# Supplementary material for: Tensor-Structured Coupled Cluster Theory
Source: arXiv:1708.02674 source file (2017-08-08)
Supplement: Supplementary file 1 [file supplementary_material.pdf]

# Supplementary Material for Tensor-Structured Coupled Cluster Theory

Roman Schutski, Jinmo Zhao, Thomas M. Henderson, and Gustavo E. Scuseria

## I. BENCHMARK CALCULATIONS

All calculations were done using standard cc-pVDZ basis set from EMSL library.[1] The errors in correlation energy were computed with respect to corresponding calculations without any approximation. The geometries of

all systems are provided in the supplemental file **geometries.zip** (they are essentially the same as in Ref. 2). For each molecule a text file is provided containing the coordinates in Angstrom. The reference energies for all calculations are given in Table I

| System                        | $E_{HF}(H)$ | $E_{c,MP2}(mH)$ | $E_{c,RCCSD}(mH)$ | $\Delta E_{c,THC-RCCSD}(mH)$ |             |
|-------------------------------|-------------|-----------------|-------------------|------------------------------|-------------|
|                               |             |                 |                   | $N_{RI}$                     | $1.5N_{RI}$ |
| Acetic acid                   | -156.107    | -156.676        | -156.728          | -156.729                     | -156.729    |
| Aniline                       | -285.758    | -953.287        | -997.193          | -998.370                     | -997.664    |
| B <sub>2</sub> F <sub>4</sub> | -447.377    | -895.977        | -909.944          | -910.646                     | -910.660    |
| Benzene                       | -230.722    | -783.594        | -823.101          | -824.086                     | -823.551    |
| Butadiene                     | -154.934    | -534.821        | -581.340          | -582.051                     | -581.615    |
| Cyclobutane                   | -156.107    | -569.106        | -621.099          | -621.994                     | -621.389    |
| Dimethylsulfoxide             | -551.556    | -618.054        | -661.870          | -661.676                     | -662.495    |
| Furan                         | -228.642    | -709.211        | -736.463          | -737.328                     | -736.917    |
| Isobutane                     | -157.310    | -590.639        | -652.505          | -653.382                     | -652.769    |
| Methylformate                 | -227.804    | -640.136        | -666.805          | -667.390                     | -667.260    |
| Methylnitrite                 | -243.681    | -690.063        | -708.990          | -709.466                     | -709.482    |
| Phenol                        | -305.586    | -967.070        | -1005.727         | -1006.614                    | -1006.241   |
| Pyridine                      | -246.714    | -809.262        | -842.453          | -843.498                     | -842.927    |
| Pyrrole                       | -208.828    | -697.260        | -727.051          | -727.907                     | -727.458    |
| Thiophene                     | -551.320    | -663.105        | -695.593          | -696.606                     | -696.250    |
| Toluene                       | -269.761    | -929.093        | -980.030          | -981.301                     | -980.491    |

TABLE I. Calculations for medium size systems

## II. COST FUNCTION

We provide expressions for a gradient of the THC objective function in Sections IV A - IV D, which is a starting point for Alternating Least Squares and Quasi-Newton methods, as described in the Section III D 2 and Eqns. 19 and 20 in the main text.

All of the provided expressions were generated by Drudge[3, 4], a computer algebra system developed in our group. The evaluation of gradient has a  $O(N^4 r_{THC})$  scaling if the tensor to be decomposed is dense, and  $O(N^2 r_{RI} r_{THC})$  scaling if the RI or SVD decomposition of the original tensor  $V$  is used. The dominant contribution to scaling originates from the contraction of  $V$  with THC factor matrices. All intermediate expressions are listed along with their corresponding scaling. Here we denote the dimension of the tensor  $V$  by  $N$  and THC ranks by  $r_{THC}$ .

## III. FACTORIZATION OF RCCSD EQUATIONS

We also list expressions used in the implementation of the fully factorized THC-RCCSD method in Sections V - XI, as described in Section IV A of the main text.

We recall that we used THC factorization of both amplitudes and two electron interaction. The factors of the interaction are denoted by  $W^1, W^2, W^3, W^4, X$ , and the ones used in the decomposition of  ${}^2T$  amplitude by  $Y^1, Y^2, Y^3, Y^4, Z$ . We use a polyadic decomposition of the energy denominator  ${}^2D$ , defined as  ${}^2D_{aibj} = \frac{1}{f_a^a - f_i^i + f_b^b - f_j^j}$ . The indices of the summations run over appropriate ranges with the specified sizes:  $O$  - occupied orbitals (size  $N_o$ ),  $V$  - virtual orbitals (size  $N_v$ ),  $A$  - auxiliary range in the THC decomposition of  ${}^2T$  amplitudes (size  $r_T$ ),  $B$  - auxiliary range in the THC decomposition of electron interaction (size  $r_V$ ),  $D$  - auxiliary range in the polyadic decomposition of energy denominator (size  $r_D$ ).

Expressions for the energy and  ${}^1T$  amplitudes are

analogs of the corresponding equations in classical RCCSD theory, although the THC structure of  ${}^2T$  amplitudes and two body interaction tensor provides a way to form intermediates with the quartic scaling of cost.

For the factors of  ${}^2T$  amplitudes we list the contractions of the doubles residuals  ${}^2R$  with the corresponding derivatives of  ${}^2T$  with respect to each factor multiplied by the denominator. For example, for the  $Y^1$  factor we list the following expression:

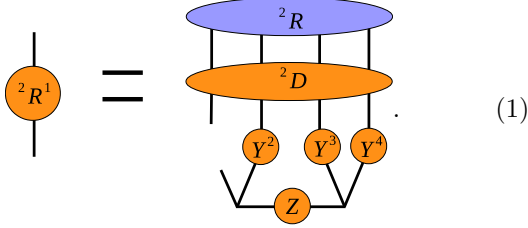

$$(1)$$

To calculate the update for the  $Y^1$  factor this diagram has to be multiplied by the inverse of the environment  $A^1$  of  $Y^1$  in  $\frac{\partial^2 T}{\partial Y^1} \cdot {}^2T$  and added the value of  $Y^1$  on the previous step:

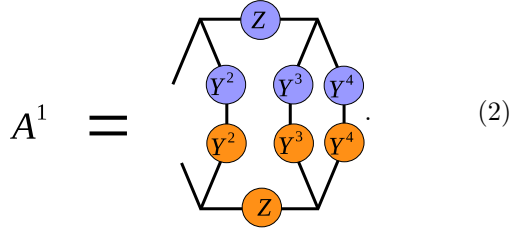

$$(2)$$

$$Y^1 \leftarrow {}^2R^1 \cdot A^{1\dagger} + Y^1 \quad (3)$$

The expressions for the environments of  $Y^1$ - $Y^4$  factors are shown in Sections XII to XVII. We note that the environment of the factor  $Z$  consists of two disjoint parts (i.e. is an outer product of two matrices), shown on the diagram below. The inverses of those parts can be calculated independently.

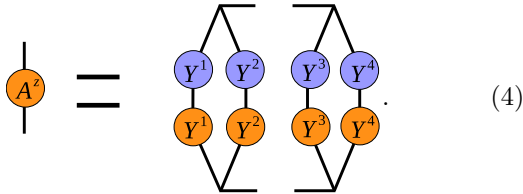

$$(4)$$

All of the listed contractions are also provided as simple Python functions and can be found in the **source\_code.zip** file. The code uses an *einsum* function from the NumPy package[5].

## IV. COST FUNCTION AND ITS GRADIENT

### A. Cost function with full tensor

$$\tau^0_{\alpha,a,b} = \sum_{c \in V} \sum_{d \in V} W^1_{c,\alpha} W^2_{d,\alpha} V^*_{c,d,a,b} \quad (3N^4 r_{THC}) \quad (5)$$

$$\tau^1_{\alpha,a} = \sum_{r \in A} \sum_{b \in V} W^3_{b,\alpha} X_{r,\alpha} \tau^0_{r,b,a} \quad (3N^2 r_{THC}^2) \quad (6)$$

$$\tau^2_{\alpha,r} = \sum_{a \in V} W^3_{a,\alpha} W^{3*}_{a,r} \quad (2N r_{THC}^2) \quad (7)$$

$$\tau^3_{\alpha,r} = \sum_{a \in V} W^4_{a,\alpha} W^{4*}_{a,r} \quad (2N r_{THC}^2) \quad (8)$$

$$\tau^4_{\alpha,r} = \sum_{\beta \in A} X_{r,\beta} \tau^2_{\beta,\alpha} \tau^3_{\beta,\alpha} \quad (3r_{THC}^3) \quad (9)$$

$$\tau^5_{\alpha,a,b} = - \sum_{c \in V} \sum_{d \in V} W^{3*}_{c,\alpha} W^{4*}_{d,\alpha} V_{a,b,c,d} \quad (3N^4 r_{THC}) \quad (10)$$

$$+ \sum_{r \in A} W^1_{a,r} W^2_{b,r} \tau^4_{\alpha,r} \quad (3N^2 r_{THC}^2) \quad (11)$$

$$\tau^6_{\alpha,a,b} = - \sum_{r \in A} X^*_{\alpha,r} \tau^5_{r,a,b} \quad (2N^2 r_{THC}^2) \quad (12)$$

$$\tau^7_{\alpha,a} = \sum_{b \in V} W^{1*}_{b,\alpha} \tau^6_{\alpha,b,a} \quad (2N^2 r_{THC}) \quad (13)$$

$$f = - \sum_{\alpha \in A} \sum_{a \in V} W^4_{a,\alpha} \tau^1_{\alpha,a} \quad (2N r_{THC}) \quad (14)$$

$$+ \sum_{a \in V} \sum_{b \in V} \sum_{c \in V} \sum_{d \in V} V_{a,b,c,d} V^*_{a,b,c,d} \quad (2N^4) \quad (15)$$

$$- \sum_{\alpha \in A} \sum_{a \in V} W^{2*}_{a,\alpha} \tau^7_{\alpha,a} \quad (2N r_{THC}) \quad (16)$$

### B. Cost function with RI decomposed tensor

$$\tau^0_{\alpha,\mu} = \sum_{a \in V} \sum_{b \in V} W^1_{a,\alpha} W^2_{b,\alpha} U^*_{L,a,b,\mu} \quad (3N^2 r_{RI} r_{THC}) \quad (17)$$

### C. Gradient of the cost function with full tensor

$$\tau_{\alpha,a,b}^1 = \sum_{\mu \in B} \tau_{\alpha,\mu}^0 U_{R,\alpha}^* U_{R,b,\mu} \quad (2N^2 r_{RI} r_{THC}) \quad (18)$$

$$\tau_{\alpha,a}^2 = \sum_{r \in A} \sum_{b \in V} W_{b,\alpha}^4 X_{\gamma,\alpha} \tau_{\gamma,a,b}^1 \quad (3N^2 r_{THC}^2) \quad (19)$$

$$\tau_{a,b,c,d}^3 = \sum_{\mu \in B} U_{L,a,b,\mu}^* U_{R,c,d,\mu} \quad (2N^4 r_{RI}) \quad (20)$$

$$\tau_{a,b,c,d}^4 = \sum_{\mu \in B} U_{L,a,b,\mu} U_{R,c,d,\mu} \quad (2N^4 r_{RI}) \quad (21)$$

$$\tau_{\alpha,\mu}^5 = \sum_{a \in V} \sum_{b \in V} W_{a,\alpha}^{1*} W_{b,\alpha}^{2*} U_{L,a,b,\mu} \quad (3N^2 r_{RI} r_{THC}) \quad (22)$$

$$\tau_{\alpha,r}^6 = \sum_{a \in V} W_{a,\alpha}^1 W_{a,r}^{1*} \quad (2N r_{THC}^2) \quad (23)$$

$$\tau_{\alpha,r}^7 = \sum_{a \in V} W_{a,\alpha}^2 W_{a,r}^{2*} \quad (2N r_{THC}^2) \quad (24)$$

$$\tau_{\alpha,r}^8 = \sum_{\beta \in A} X_{\beta,r} \tau_{\beta,\alpha}^6 \tau_{\beta,\alpha}^7 \quad (3r_{THC}^3) \quad (25)$$

$$\tau_{\alpha,a,b}^9 = \sum_{\mu \in B} \tau_{\alpha,\mu}^5 U_{R,a,b,\mu} \quad (2N^2 r_{RI} r_{THC}) \quad (26)$$

$$- \sum_{\gamma \in A} W_{a,r}^3 W_{b,r}^4 \tau_{\alpha,r}^8 \quad (3N^2 r_{THC}^2) \quad (27)$$

$$\tau_{\alpha,\gamma,a}^{10} = \sum_{b \in V} W_{b,\alpha}^{3*} \tau_{\alpha,b,a}^9 \quad (2N^2 r_{THC}^2) \quad (28)$$

$$\tau_{\alpha,r}^{11} = \sum_{a \in V} W_{a,r}^{4*} \tau_{\alpha,\gamma,a}^{10} \quad (2N r_{THC}^2) \quad (29)$$

$$f = - \sum_{\alpha \in A} \sum_{a \in V} W_{a,\alpha}^3 \tau_{\alpha,a}^2 \quad (2N r_{THC}) \quad (30)$$

$$+ \sum_{a \in V} \sum_{b \in V} \sum_{c \in V} \sum_{d \in V} \tau_{a,b,c,d}^3 \tau_{a,b,c,d}^4 \quad (2N^4) \quad (31)$$

$$- \sum_{\alpha \in A} \sum_{\gamma \in A} X_{\alpha,r}^* \tau_{\alpha,r}^{11} \quad (2r_{THC}^2) \quad (32)$$

$$\tau_{\alpha,\gamma}^0 = \sum_{a \in V} W_{a,\alpha}^3 W_{a,\gamma}^{3*} \quad (2N r_{THC}^2) \quad (33)$$

$$\tau_{\alpha,\gamma}^1 = \sum_{a \in V} W_{a,\alpha}^4 W_{a,\gamma}^{4*} \quad (2N r_{THC}^2) \quad (34)$$

$$\tau_{\alpha,\gamma}^2 = \sum_{\alpha 0 \in A} X_{\gamma,\beta}^* \tau_{\alpha,\beta}^0 \tau_{\alpha,\beta}^1 \quad (3r_{THC}^3) \quad (35)$$

$$\tau_{\alpha,a,b}^3 = \sum_{\gamma \in A} W_{a,\gamma}^{1*} W_{b,\gamma}^{2*} \tau_{\alpha,\gamma}^2 \quad (3N^2 r_{THC}^2) \quad (36)$$

$$- \sum_{c \in V} \sum_{d \in V} W_{c,\alpha}^3 W_{d,\alpha}^4 V_{c,a,b,c,d} \quad (3N^4 r_{THC}) \quad (37)$$

$$\tau_{\alpha,a,b}^4 = - \sum_{\gamma \in A} X_{\alpha,\gamma} \tau_{\gamma,a,b}^3 \quad (2N^2 r_{THC}^2) \quad (38)$$

$$\frac{\partial f}{\partial W_{a,\alpha}^1} = - \sum_{b \in V} W_{b,\alpha}^2 \tau_{\alpha,a,b}^4 \quad (2N^2 r_{THC}) \quad (39)$$

$$\tau_{\alpha,\gamma}^0 = \sum_{a \in V} W_{a,\alpha}^3 W_{a,\gamma}^{3*} \quad (2N r_{THC}^2) \quad (40)$$

$$\tau_{\alpha,\gamma}^1 = \sum_{a \in V} W_{a,\alpha}^4 W_{a,\gamma}^{4*} \quad (2N r_{THC}^2) \quad (41)$$

$$\tau_{\alpha,\gamma}^2 = \sum_{\alpha 0 \in A} X_{\gamma,\beta}^* \tau_{\alpha,\beta}^0 \tau_{\alpha,\beta}^1 \quad (3r_{THC}^3) \quad (42)$$

$$\tau_{\alpha,a,b}^3 = \sum_{\gamma \in A} W_{a,\gamma}^{1*} W_{b,\gamma}^{2*} \tau_{\alpha,\gamma}^2 \quad (3N^2 r_{THC}^2) \quad (43)$$

$$- \sum_{c \in V} \sum_{d \in V} W_{c,\alpha}^3 W_{d,\alpha}^4 V_{c,a,b,c,d} \quad (3N^4 r_{THC}) \quad (44)$$

$$\tau_{\alpha,a,b}^4 = - \sum_{\gamma \in A} X_{\alpha,\gamma} \tau_{\gamma,a,b}^3 \quad (2N^2 r_{THC}^2) \quad (45)$$

$$\frac{\partial f}{\partial W_{a,\alpha}^2} = - \sum_{b \in V} W_{b,\alpha}^1 \tau_{\alpha,a,b}^4 \quad (2N^2 r_{THC}) \quad (46)$$

$$\tau^0_{\alpha,\gamma} = \sum_{a \in V} W^1_{a,\alpha} W^{1*}_{a,\gamma} \quad (2Nr_{THC}^2) \quad (47)$$

$$\tau^1_{\alpha,\gamma} = \sum_{a \in V} W^2_{a,\alpha} W^{2*}_{a,\gamma} \quad (2Nr_{THC}^2) \quad (48)$$

$$\tau^2_{\alpha,\gamma} = \sum_{\alpha 0 \in A} X^*_{\beta,\gamma} \tau^0_{\alpha,\beta} \tau^1_{\alpha,\gamma} \quad (3r_{THC}^3) \quad (49)$$

$$\begin{aligned} \tau^3_{\alpha,a,b} &= \sum_{c \in V} \sum_{d \in V} W^1_{c,\alpha} W^2_{d,\alpha} V c_{c,d,a,b} \quad (3N^4 r_{THC}) \\ &\quad - \sum_{\gamma \in A} W^{3*}_{a,\gamma} W^{4*}_{b,\gamma} \tau^2_{\alpha,\gamma} \quad (3N^2 r_{THC}^2) \end{aligned} \quad (50)$$

$$(51)$$

$$\tau^4_{\alpha,\gamma,a} = \sum_{b \in V} W^3_{b,\gamma} \tau^3_{\alpha,b,a} \quad (2N^2 r_{THC}^2) \quad (52)$$

$$\frac{\partial f}{\partial X_{\alpha,\gamma}} = - \sum_{a \in V} W^4_{a,\gamma} \tau^4_{\alpha,\gamma,a} \quad (2Nr_{THC}^2) \quad (53)$$

$$\tau^0_{\alpha,\gamma} = \sum_{a \in V} W^1_{a,\alpha} W^{1*}_{a,\gamma} \quad (2Nr_{THC}^2) \quad (54)$$

$$\tau^1_{\alpha,\gamma} = \sum_{a \in V} W^2_{a,\alpha} W^{2*}_{a,\gamma} \quad (2Nr_{THC}^2) \quad (55)$$

$$\tau^2_{\alpha,\gamma} = \sum_{\alpha 0 \in A} X^*_{\beta,\gamma} \tau^0_{\alpha,\beta} \tau^1_{\alpha,\gamma} \quad (3r_{THC}^3) \quad (56)$$

$$\begin{aligned} \tau^3_{\alpha,a,b} &= \sum_{\gamma \in A} W^{3*}_{a,\gamma} W^{4*}_{b,\gamma} \tau^2_{\alpha,\gamma} \quad (3N^2 r_{THC}^2) \\ &\quad - \sum_{c \in V} \sum_{d \in V} W^1_{c,\alpha} W^2_{d,\alpha} V c_{c,d,a,b} \quad (3N^4 r_{THC}) \end{aligned} \quad (57)$$

$$(58)$$

$$\tau^4_{\alpha,a,b} = - \sum_{\gamma \in A} X_{\gamma,\alpha} \tau^3_{\gamma,a,b} \quad (2N^2 r_{THC}^2) \quad (59)$$

$$\frac{\partial f}{\partial W^3_{a,\alpha}} = - \sum_{b \in V} W^4_{b,\alpha} \tau^4_{\alpha,a,b} \quad (2N^2 r_{THC}) \quad (60)$$

$$\tau^0_{\alpha,\gamma} = \sum_{a \in V} W^1_{a,\alpha} W^{1*}_{a,\gamma} \quad (2Nr_{THC}^2) \quad (61)$$

$$\tau^1_{\alpha,\gamma} = \sum_{a \in V} W^2_{a,\alpha} W^{2*}_{a,\gamma} \quad (2Nr_{THC}^2) \quad (62)$$

$$\tau^2_{\alpha,\gamma} = \sum_{\alpha 0 \in A} X^*_{\beta,\gamma} \tau^0_{\alpha,\beta} \tau^1_{\alpha,\gamma} \quad (3r_{THC}^3) \quad (63)$$

$$\begin{aligned} \tau^3_{\alpha,a,b} &= \sum_{\gamma \in A} W^{3*}_{a,\gamma} W^{4*}_{b,\gamma} \tau^2_{\alpha,\gamma} \quad (3N^2 r_{THC}^2) \\ &\quad - \sum_{c \in V} \sum_{d \in V} W^1_{c,\alpha} W^2_{d,\alpha} V c_{c,d,a,b} \quad (3N^4 r_{THC}) \end{aligned} \quad (64)$$

$$(65)$$

$$\tau^4_{\alpha,a,b} = - \sum_{\gamma \in A} X_{\gamma,\alpha} \tau^3_{\gamma,a,b} \quad (2N^2 r_{THC}^2) \quad (66)$$

$$\frac{\partial f}{\partial W^4_{a,\alpha}} = - \sum_{b \in V} W^3_{b,\alpha} \tau^4_{\alpha,b,a} \quad (2N^2 r_{THC}) \quad (67)$$

#### D. Gradient of the cost function with RI decomposed tensor

$$\tau^0_{\alpha,\gamma} = \sum_{a \in V} W^2_{a,\alpha} W^{2*}_{a,\gamma} \quad (2Nr_{THC}^2) \quad (68)$$

$$\tau^1_{\alpha,\gamma} = \sum_{a \in V} W^3_{a,\alpha} W^{3*}_{a,\gamma} \quad (2Nr_{THC}^2) \quad (69)$$

$$\tau^2_{\alpha,\gamma} = \sum_{a \in V} W^4_{a,\alpha} W^{4*}_{a,\gamma} \quad (2Nr_{THC}^2) \quad (70)$$

$$\tau^3_{\alpha,\gamma} = \sum_{\beta \in A} X c_{r,\beta} \tau^1_{\alpha,\beta} \tau^2_{\alpha,\gamma} \quad (3r_{THC}^3) \quad (71)$$

$$\tau^4_{\alpha,\gamma} = \sum_{\beta \in A} X_{\alpha,\beta} \tau^3_{\beta,\gamma} \quad (2r_{THC}^3) \quad (72)$$

$$\tau^5_{\alpha,w,a} = \sum_{b \in V} W^4_{b,\alpha} U_R^*_{a,b,w} \quad (2N^2 r_{RI} r_{THC}) \quad (73)$$

$$\tau^6_{\alpha,w} = \sum_{a \in V} W^3_{a,\alpha} \tau^5_{\alpha,w,a} \quad (2Nr_{RI}r_{THC}) \quad (74)$$

$$\tau^7_{\alpha,w} = \sum_{\gamma \in A} X_{\alpha,\gamma} \tau^6_{r,w} \quad (2r_{RI}r_{THC}^2) \quad (75)$$

$$\frac{\partial f}{\partial W^1_{a,\alpha}} = \sum_{\gamma \in A} W^{1*}_{a,\gamma} \tau^0_{\alpha,\gamma} \tau^4_{\alpha,\gamma} \quad (3Nr_{THC}^2) \quad (76)$$

$$- \sum_{w \in B} \sum_{b \in V} W^2_{b,\alpha} \tau^7_{\alpha,w} U_L^*_{a,b,w} \quad (3N^2r_{RI}r_{THC}) \quad (77)$$

$$\tau^0_{\alpha,\gamma} = \sum_{a \in V} W^1_{a,\alpha} W^{1*}_{a,\gamma} \quad (2Nr_{THC}^2) \quad (78)$$

$$\tau^1_{\alpha,\gamma} = \sum_{a \in V} W^3_{a,\alpha} W^{3*}_{a,\gamma} \quad (2Nr_{THC}^2) \quad (79)$$

$$\tau^2_{\alpha,\gamma} = \sum_{a \in V} W^4_{a,\alpha} W^{4*}_{a,\gamma} \quad (2Nr_{THC}^2) \quad (80)$$

$$\tau^3_{\alpha,\gamma} = \sum_{\beta \in A} X_{c_{r,\beta}} \tau^1_{\alpha,\beta} \tau^2_{\alpha,\beta} \quad (3r_{THC}^3) \quad (81)$$

$$\tau^4_{\alpha,\gamma} = \sum_{\beta \in A} X_{\alpha,\beta} \tau^3_{\beta,\gamma} \quad (2r_{THC}^3) \quad (82)$$

$$\tau^5_{\alpha,w,a} = \sum_{b \in V} W^4_{b,\alpha} U_R^*_{a,b,w} \quad (2N^2r_{RI}r_{THC}) \quad (83)$$

$$\tau^6_{\alpha,w} = \sum_{a \in V} W^3_{a,\alpha} \tau^5_{\alpha,w,a} \quad (2Nr_{RI}r_{THC}) \quad (84)$$

$$\tau^7_{\alpha,w} = \sum_{\gamma \in A} X_{\alpha,\gamma} \tau^6_{r,w} \quad (2r_{RI}r_{THC}^2) \quad (85)$$

$$\frac{\partial f}{\partial W^2_{a,\alpha}} = \sum_{\gamma \in A} W^{2*}_{a,\gamma} \tau^0_{\alpha,\gamma} \tau^4_{\alpha,\gamma} \quad (3Nr_{THC}^2) \quad (86)$$

$$- \sum_{w \in B} \sum_{b \in V} W^1_{b,\alpha} \tau^7_{\alpha,w} U_L^*_{b,a,w} \quad (3N^2r_{RI}r_{THC}) \quad (87)$$

$$\tau^0_{\alpha,w,a} = \sum_{b \in V} W^2_{b,\alpha} U_L^*_{a,b,w} \quad (2N^2r_{RI}r_{THC}) \quad (88)$$

$$\tau^1_{\alpha,w} = \sum_{a \in V} W^1_{a,\alpha} \tau^0_{\alpha,w,a} \quad (2Nr_{RI}r_{THC}) \quad (89)$$

$$\tau^2_{\alpha,w,a} = \sum_{b \in V} W^4_{b,\alpha} U_R^*_{a,b,w} \quad (2N^2r_{RI}r_{THC}) \quad (90)$$

$$\tau^3_{\alpha,w} = \sum_{a \in V} W^3_{a,\alpha} \tau^2_{\alpha,w,a} \quad (2Nr_{RI}r_{THC}) \quad (91)$$

$$\tau^4_{\alpha,\gamma} = \sum_{a \in V} W^1_{a,\alpha} W^{1*}_{a,\gamma} \quad (2Nr_{THC}^2) \quad (92)$$

$$\tau^5_{\alpha,\gamma} = \sum_{a \in V} W^2_{a,\alpha} W^{2*}_{a,\gamma} \quad (2Nr_{THC}^2) \quad (93)$$

$$\tau^6_{\alpha,\gamma} = \sum_{a \in V} W^3_{a,\alpha} W^{3*}_{a,\gamma} \quad (2Nr_{THC}^2) \quad (94)$$

$$\tau^7_{\alpha,\gamma} = \sum_{a \in V} W^4_{a,\alpha} W^{4*}_{a,\gamma} \quad (2Nr_{THC}^2) \quad (95)$$

$$\tau^8_{\alpha,\gamma} = \sum_{\beta \in A} X_{c_{r,\beta}} \tau^6_{\alpha,\beta} \tau^7_{\alpha,\beta} \quad (3r_{THC}^3) \quad (96)$$

$$\frac{\partial f}{\partial X_{\alpha,\gamma}} = - \sum_{w \in B} \tau^1_{\alpha,w} \tau^3_{r,w} \quad (2r_{RI}r_{THC}^2) \quad (97)$$

$$+ \sum_{\beta \in A} \tau^4_{\alpha,\beta} \tau^5_{\alpha,\beta} \tau^8_{r,\beta} \quad (3r_{THC}^3) \quad (98)$$

$$\tau^0_{\alpha,\gamma} = \sum_{a \in V} W^1_{a,\alpha} W^{1*}_{a,\gamma} \quad (2Nr_{THC}^2) \quad (99)$$

$$\tau^1_{\alpha,\gamma} = \sum_{a \in V} W^2_{a,\alpha} W^{2*}_{a,\gamma} \quad (2Nr_{THC}^2) \quad (100)$$

$$\tau^2_{\alpha,\gamma} = \sum_{\beta \in A} X_{c_{\beta,\gamma}} \tau^0_{\alpha,\beta} \tau^1_{\alpha,\beta} \quad (3r_{THC}^3) \quad (101)$$

$$\tau^3_{\alpha,\gamma} = \sum_{\beta \in A} X_{\beta,\alpha} \tau^2_{\beta,\gamma} \quad (2r_{THC}^3) \quad (102)$$

## V. THC-RCCSD ENERGY

Here expressions for a THC-RCCSD energy are given along with their cost

$$\tau_{\alpha,\gamma}^4 = \sum_{a \in V} W_{a,\alpha}^4 W_{a,\gamma}^{4*} \quad (2Nr_{THC}^2) \quad (103)$$

$$\tau_{\alpha,w,a}^5 = \sum_{b \in V} W_{b,\alpha}^2 U_{L,a,b,w}^* \quad (2N^2 r_{RI} r_{THC}) \quad (104)$$

$$\tau_{\alpha,w}^6 = \sum_{a \in V} W_{a,\alpha}^1 \tau_{\alpha,w,a}^5 \quad (2Nr_{RI} r_{THC}) \quad (105)$$

$$\tau_{\alpha,w}^7 = \sum_{\gamma \in A} X_{r,\alpha} \tau_{r,w}^6 \quad (2r_{RI} r_{THC}^2) \quad (106)$$

$$\frac{\partial f}{\partial W_{a,\alpha}^3} = \sum_{\gamma \in A} W_{a,\gamma}^{3*} \tau_{\alpha,\gamma}^3 \tau_{\alpha,\gamma}^4 \quad (3Nr_{THC}^2) \quad (107)$$

$$- \sum_{w \in B} \sum_{b \in V} W_{b,\alpha}^4 \tau_{\alpha,w}^7 U_{R,a,b,w}^* \quad (3N^2 r_{RI} r_{THC}) \quad (108)$$

$$\tau_{\alpha,\gamma}^0 = \sum_{a \in V} W_{a,\alpha}^1 W_{a,\gamma}^{1*} \quad (2Nr_{THC}^2) \quad (109)$$

$$\tau_{\alpha,\gamma}^1 = \sum_{a \in V} W_{a,\alpha}^2 W_{a,\gamma}^{2*} \quad (2Nr_{THC}^2) \quad (110)$$

$$\tau_{\alpha,\gamma}^2 = \sum_{\beta \in A} X_{\beta,\gamma} \tau_{\alpha,\beta}^0 \tau_{\alpha,\beta}^1 \quad (3r_{THC}^3) \quad (111)$$

$$\tau_{\alpha,\gamma}^3 = \sum_{\beta \in A} X_{\beta,\alpha} \tau_{\beta,\gamma}^2 \quad (2r_{THC}^3) \quad (112)$$

$$\tau_{\alpha,\gamma}^4 = \sum_{a \in V} W_{a,\alpha}^3 W_{a,\gamma}^{3*} \quad (2Nr_{THC}^2) \quad (113)$$

$$\tau_{\alpha,w,a}^5 = \sum_{b \in V} W_{b,\alpha}^2 U_{L,a,b,w}^* \quad (2N^2 r_{RI} r_{THC}) \quad (114)$$

$$\tau_{\alpha,w}^6 = \sum_{a \in V} W_{a,\alpha}^1 \tau_{\alpha,w,a}^5 \quad (2Nr_{RI} r_{THC}) \quad (115)$$

$$\tau_{\alpha,w}^7 = \sum_{\gamma \in A} X_{r,\alpha} \tau_{r,w}^6 \quad (2r_{RI} r_{THC}^2) \quad (116)$$

$$\frac{\partial f}{\partial W_{a,\alpha}^4} = \sum_{\gamma \in A} W_{a,\gamma}^{4*} \tau_{\alpha,\gamma}^3 \tau_{\alpha,\gamma}^4 \quad (3Nr_{THC}^2) \quad (117)$$

$$- \sum_{w \in B} \sum_{b \in V} W_{b,\alpha}^3 \tau_{\alpha,w}^7 U_{R,a,b,w}^* \quad (3N^2 r_{RI} r_{THC}) \quad (118)$$

### A. Contributions from $(H^1 T)_c$

Raw expression

$$E \leftarrow \sum_{i \in O} \sum_{a \in V} 2^1 T_{a,i} f_{i,a} \quad (119)$$

Factorized expression

$$E \leftarrow \sum_{i \in O} \sum_{a \in V} 2^1 T_{a,i} f_{i,a} \quad (2N_o N_v) \quad (120)$$

### B. Contributions from $(H^1 T^1 T)_c$

Raw expression

$$E \leftarrow - \sum_{\alpha \in B} \sum_{\beta \in B} \sum_{i \in O} \sum_{j \in O} \sum_{a \in V} \sum_{b \in V} 1 T_{a,j} 1 T_{b,i} W_{i,\alpha}^1 W_{a,\alpha}^2 X_{\alpha,\beta} W_{j,\beta}^3 W_{b,\beta}^4 \quad (121)$$

Factorized expression

$$\tau_{\alpha,i}^0 = \sum_{a \in V} 1 T_{a,i} W_{a,\alpha}^2 \quad (2r_V N_o N_v) \quad (122)$$

$$\tau_{\alpha,\beta}^1 = \sum_{i \in O} W_{i,\beta}^3 \tau_{\alpha,i}^0 \quad (2r_V^2 N_o) \quad (123)$$

$$\tau_{\alpha,i}^2 = \sum_{\beta \in B} W_{i,\beta}^1 X_{\beta,\alpha} \tau_{\beta,\alpha}^1 \quad (3r_V^2 N_o) \quad (124)$$

$$\tau_{i,a}^3 = \sum_{\alpha \in B} W_{a,\alpha}^4 \tau_{\alpha,i}^2 \quad (2r_V N_o N_v) \quad (125)$$

$$E \leftarrow - \sum_{i \in O} \sum_{a \in V} 1 T_{a,i} \tau_{i,a}^3 \quad (2N_o N_v) \quad (126)$$

Raw expression

$$E \leftarrow \sum_{\alpha \in B} \sum_{\beta \in B} \sum_{i \in O} \sum_{j \in O} \sum_{a \in V} \sum_{b \in V} 2^1 T_{a,i} 1 T_{b,j} W_{i,\alpha}^1 W_{a,\alpha}^2 X_{\alpha,\beta} W_{j,\beta}^3 W_{b,\beta}^4 \quad (127)$$

Factorized expression

$$\tau^0_{\alpha,i} = \sum_{a \in V} {}^1T_{a,i} W^2_{a,\alpha} \quad (2r_V N_o N_v) \quad (128)$$

$$\tau^1_{\alpha} = \sum_{i \in O} W^1_{i,\alpha} \tau^0_{\alpha,i} \quad (2r_V N_o) \quad (129)$$

$$\tau^2_{\alpha} = \sum_{\beta \in B} \tau^1_{\beta} X_{\beta,\alpha} \quad (2r_V^2) \quad (130)$$

$$\tau^3_{i,a} = \sum_{\alpha \in B} \tau^2_{\alpha} W^3_{i,\alpha} W^4_{a,\alpha} \quad (3r_V N_o N_v) \quad (131)$$

$$E \leftarrow \sum_{i \in O} \sum_{a \in V} 2 {}^1T_{a,i} \tau^3_{i,a} \quad (2N_o N_v) \quad (132)$$

### C. Contributions from $(H^2T)_c$

Raw expression

$$E \leftarrow - \sum_{\gamma \in A} \sum_{\delta \in A} \sum_{\alpha \in B} \sum_{\beta \in B} \sum_{i \in O} \sum_{j \in O} \sum_{a \in V} \sum_{b \in V} W^1_{i,\alpha} W^2_{a,\alpha} X_{\alpha,\beta} W^3_{j,\beta} W^4_{b,\beta} Y^1_{b,\gamma} Y^2_{i,\gamma} Z_{\gamma,\delta} Y^3_{a,\delta} Y^4_{j,\delta} \quad (133)$$

Factorized expression

$$\tau^0_{\gamma,\alpha} = \sum_{a \in V} W^4_{a,\alpha} Y^1_{a,\gamma} \quad (2r_T r_V N_v) \quad (134)$$

$$\tau^1_{\gamma,\alpha} = \sum_{i \in O} W^3_{i,\alpha} Y^4_{i,\gamma} \quad (2r_T r_V N_o) \quad (135)$$

$$\tau^2_{\gamma,\alpha} = \sum_{i \in O} W^1_{i,\alpha} Y^2_{i,\gamma} \quad (2r_T r_V N_o) \quad (136)$$

$$\tau^3_{\gamma,\alpha} = \sum_{a \in V} W^2_{a,\alpha} Y^3_{a,\gamma} \quad (2r_T r_V N_v) \quad (137)$$

$$\tau^4_{\alpha,\beta} = \sum_{\gamma \in A} \sum_{\delta \in A} Z_{\gamma,\delta} \tau^0_{\gamma,\beta} \tau^1_{\delta,\beta} \tau^2_{\gamma,\alpha} \tau^3_{\delta,\alpha} \quad (5r_T^2 r_V^2) \quad (138)$$

$$E \leftarrow - \sum_{\alpha \in B} \sum_{\beta \in B} X_{\alpha,\beta} \tau^4_{\alpha,\beta} \quad (2r_V^2) \quad (139)$$

Raw expression

$$E \leftarrow \sum_{\gamma \in A} \sum_{\delta \in A} \sum_{\alpha \in B} \sum_{\beta \in B} \sum_{i \in O} \sum_{j \in O} \sum_{a \in V} \sum_{b \in V} 2 W^1_{i,\alpha} W^2_{a,\alpha} X_{\alpha,\beta} W^3_{j,\beta} W^4_{b,\beta} Y^1_{a,\gamma} Y^2_{i,\gamma} Z_{\gamma,\delta} Y^3_{b,\delta} Y^4_{j,\delta} \quad (140)$$

Factorized expression

$$\tau^0_{\gamma,\alpha} = \sum_{a \in V} W^4_{a,\alpha} Y^3_{a,\gamma} \quad (2r_T r_V N_v) \quad (141)$$

$$\tau^1_{\gamma,\alpha} = \sum_{i \in O} W^3_{i,\alpha} Y^4_{i,\gamma} \quad (2r_T r_V N_o) \quad (142)$$

$$\tau^2_{\gamma,\alpha} = \sum_{\beta \in B} X_{\alpha,\beta} \tau^0_{\gamma,\beta} \tau^1_{\gamma,\beta} \quad (3r_T r_V^2) \quad (143)$$

$$\tau^3_{\gamma,\alpha} = \sum_{a \in V} W^2_{a,\alpha} Y^1_{a,\gamma} \quad (2r_T r_V N_v) \quad (144)$$

$$\tau^4_{\gamma,\alpha} = \sum_{i \in O} W^1_{i,\alpha} Y^2_{i,\gamma} \quad (2r_T r_V N_o) \quad (145)$$

$$\tau^5_{\gamma,\delta} = \sum_{\alpha \in B} \tau^2_{\delta,\alpha} \tau^3_{\gamma,\alpha} \tau^4_{\gamma,\alpha} \quad (3r_T^2 r_V) \quad (146)$$

$$E \leftarrow \sum_{\gamma \in A} \sum_{\delta \in A} 2 Z_{\gamma,\delta} \tau^5_{\gamma,\delta} \quad (2r_T^2) \quad (147)$$

## VI. THC-RCCSD ${}^1R$ EQUATION

Here expressions for a THC-RCCSD singles residual are given along with their cost

### A. Contributions from $H$

Raw expression

$${}^1R_{a,i} \leftarrow f_{a,i} \quad (148)$$

Factorized expression

$${}^1R_{a,i} \leftarrow f_{a,i} \quad (0) \quad (149)$$

### B. Contributions from $(H^1 T)_c$

Raw expression

$${}^1R_{a,i} \leftarrow - \sum_{j \in O} {}^1T_{a,j} f_{j,i} \quad (150)$$

Factorized expression

$${}^1R_{a,i} \leftarrow - \sum_{j \in O} {}^1T_{a,j} f_{j,i} \quad (2N_o^2 N_v) \quad (151)$$

Raw expression

$${}^1R_{a,i} \leftarrow - \sum_{j \in O} \sum_{b \in V} {}^1T_{b,j} V_{a,b,j,i} \quad (152)$$

Factorized expression

$$\tau^0_{\alpha,i} = \sum_{a \in V} {}^1T_{a,i} W^2_{a,\alpha} \quad (2r_V N_o N_v) \quad (153)$$

$$\tau^1_{\alpha,\beta} = \sum_{i \in O} W^3_{i,\beta} \tau^0_{\alpha,i} \quad (2r_V^2 N_o) \quad (154)$$

$$\tau^2_{\alpha,i} = \sum_{\beta \in B} X_{\alpha,\beta} W^4_{i,\beta} \tau^1_{\alpha,\beta} \quad (3r_V^2 N_o) \quad (155)$$

$${}^1R_{a,i} \leftarrow - \sum_{\alpha \in B} W^1_{a,\alpha} \tau^2_{\alpha,i} \quad (2r_V N_o N_v) \quad (156)$$

Raw expression

$${}^1R_{a,i} \leftarrow \sum_{j \in O} \sum_{b \in V} 2 {}^1T_{b,j} V_{a,i,j,b} \quad (157)$$

Factorized expression

$$\tau^0_{\alpha,i} = \sum_{a \in V} {}^1T_{a,i} W^4_{a,\alpha} \quad (2r_V N_o N_v) \quad (158)$$

$$\tau^1_{\alpha} = \sum_{i \in O} W^3_{i,\alpha} \tau^0_{\alpha,i} \quad (2r_V N_o) \quad (159)$$

$$\tau^2_{\alpha} = \sum_{\beta \in B} \tau^1_{\beta} X_{\alpha,\beta} \quad (2r_V^2) \quad (160)$$

$${}^1R_{a,i} \leftarrow \sum_{\alpha \in B} 2 \tau^2_{\alpha} W^1_{a,\alpha} W^2_{i,\alpha} \quad (3r_V N_o N_v) \quad (161)$$

Raw expression

$${}^1R_{a,i} \leftarrow \sum_{b \in V} {}^1T_{b,i} f_{a,b} \quad (162)$$

Factorized expression

$${}^1R_{a,i} \leftarrow \sum_{b \in V} {}^1T_{b,i} f_{a,b} \quad (2N_o N_v^2) \quad (163)$$

### C. Contributions from $(H^1 T^1 T)_c$

Raw expression

$${}^1R_{a,i} \leftarrow - \sum_{j \in O} \sum_{b \in V} \sum_{c \in V} {}^1T_{b,i} {}^1T_{c,j} V_{a,c,j,b} \quad (164)$$

Factorized expression

$$\tau^0_{\alpha,i} = \sum_{a \in V} {}^1T_{a,i} W^2_{a,\alpha} \quad (2r_V N_o N_v) \quad (165)$$

$$\tau^1_{\alpha,\beta} = \sum_{i \in O} W^3_{i,\beta} \tau^0_{\alpha,i} \quad (2r_V^2 N_o) \quad (166)$$

$$\tau^2_{\alpha,a} = \sum_{\beta \in B} X_{\alpha,\beta} W^4_{a,\beta} \tau^1_{\alpha,\beta} \quad (3r_V^2 N_v) \quad (167)$$

$$\tau^3_{a,b} = \sum_{\alpha \in B} W^1_{a,\alpha} \tau^2_{\alpha,b} \quad (2r_V N_v^2) \quad (168)$$

$${}^1R_{a,i} \leftarrow - \sum_{b \in V} {}^1T_{b,i} \tau^3_{a,b} \quad (2N_o N_v^2) \quad (169)$$

Raw expression

$${}^1R_{a,i} \leftarrow \sum_{j \in O} \sum_{b \in V} \sum_{c \in V} 2 {}^1T_{b,i} {}^1T_{c,j} V_{a,b,j,c} \quad (170)$$

Factorized expression

$$\tau^0_{\alpha,i} = \sum_{a \in V} {}^1T_{a,i} W^4_{a,\alpha} \quad (2r_V N_o N_v) \quad (171)$$

$$\tau^1_{\alpha} = \sum_{i \in O} W^3_{i,\alpha} \tau^0_{\alpha,i} \quad (2r_V N_o) \quad (172)$$

$$\tau^2_{\alpha} = \sum_{\beta \in B} \tau^1_{\beta} X_{\alpha,\beta} \quad (2r_V^2) \quad (173)$$

$$\tau^3_{a,b} = \sum_{\alpha \in B} \tau^2_{\alpha} W^1_{a,\alpha} W^2_{b,\alpha} \quad (3r_V N_v^2) \quad (174)$$

$${}^1R_{a,i} \leftarrow \sum_{b \in V} 2 {}^1T_{b,i} \tau^3_{a,b} \quad (2N_o N_v^2) \quad (175)$$

Raw expression

$${}^1R_{a,i} \leftarrow - \sum_{j \in O} \sum_{b \in V} {}^1T_{a,j} {}^1T_{b,i} f_{j,b} \quad (176)$$



Factorized expression

$$\tau^0_{i,j} = \sum_{a \in V} {}^1T_{a,i} f_{j,a} \quad (2N_o^2 N_v) \quad (177)$$

$${}^1R_{a,i} \leftarrow - \sum_{j \in O} {}^1T_{a,j} \tau^0_{i,j} \quad (2N_o^2 N_v) \quad (178)$$

Raw expression

$${}^1R_{a,i} \leftarrow \sum_{j \in O} \sum_{k \in O} \sum_{b \in V} {}^1T_{a,j} {}^1T_{b,k} V_{k,i,j,b} \quad (179)$$

Factorized expression

$$\tau^0_{\alpha,i} = \sum_{a \in V} {}^1T_{a,i} W^4_{a,\alpha} \quad (2r_V N_o N_v) \quad (180)$$

$$\tau^1_{\alpha,\beta} = \sum_{i \in O} W^1_{i,\alpha} \tau^0_{\beta,i} \quad (2r_V^2 N_o) \quad (181)$$

$$\tau^2_{\alpha,i} = \sum_{\beta \in B} X_{\alpha,\beta} W^3_{i,\beta} \tau^1_{\alpha,\beta} \quad (3r_V^2 N_o) \quad (182)$$

$$\tau^3_{i,j} = \sum_{\alpha \in B} W^2_{i,\alpha} \tau^2_{\alpha,j} \quad (2r_V N_o^2) \quad (183)$$

$${}^1R_{a,i} \leftarrow \sum_{j \in O} {}^1T_{a,j} \tau^3_{i,j} \quad (2N_o^2 N_v) \quad (184)$$

Raw expression

$${}^1R_{a,i} \leftarrow - \sum_{j \in O} \sum_{k \in O} \sum_{b \in V} 2 {}^1T_{a,j} {}^1T_{b,k} V_{j,i,k,b} \quad (185)$$

Factorized expression

$$\tau^0_{\alpha,i} = \sum_{a \in V} {}^1T_{a,i} W^4_{a,\alpha} \quad (2r_V N_o N_v) \quad (186)$$

$$\tau^1_{\alpha} = \sum_{i \in O} W^3_{i,\alpha} \tau^0_{\alpha,i} \quad (2r_V N_o) \quad (187)$$

$$\tau^2_{\alpha} = \sum_{\beta \in B} \tau^1_{\beta} X_{\alpha,\beta} \quad (2r_V^2) \quad (188)$$

$$\tau^3_{i,j} = \sum_{\alpha \in B} \tau^2_{\alpha} W^1_{i,\alpha} W^2_{j,\alpha} \quad (3r_V N_o^2) \quad (189)$$

$${}^1R_{a,i} \leftarrow - \sum_{j \in O} 2 {}^1T_{a,j} \tau^3_{j,i} \quad (2N_o^2 N_v) \quad (190)$$

**D. Contributions from  $(H^2T)_c$**

Raw expression

$${}^1R_{a,i} \leftarrow \sum_{j \in O} \sum_{b \in V} \sum_{c \in V} {}^2T_{b,i,c,j} V_{a,b,j,c} \quad (191)$$

Factorized expression

$$\tau^0_{\gamma,\alpha} = \sum_{a \in V} W^2_{a,\alpha} Y^1_{a,\gamma} \quad (2r_T r_V N_v) \quad (192)$$

$$\tau^1_{\gamma,\alpha} = \sum_{i \in O} W^3_{i,\alpha} Y^4_{i,\gamma} \quad (2r_T r_V N_o) \quad (193)$$

$$\tau^2_{\gamma,\alpha} = \sum_{a \in V} W^4_{a,\alpha} Y^3_{a,\gamma} \quad (2r_T r_V N_v) \quad (194)$$

$$\tau^3_{\gamma,\alpha} = \sum_{\beta \in B} X_{\alpha,\beta} \tau^1_{\gamma,\beta} \tau^2_{\gamma,\beta} \quad (3r_T r_V^2) \quad (195)$$

$$\tau^4_{\gamma,\alpha} = \sum_{\delta \in A} Z_{\gamma,\delta} \tau^3_{\delta,\alpha} \quad (2r_T^2 r_V) \quad (196)$$

$$\tau^5_{\gamma,a} = \sum_{\alpha \in B} W^1_{a,\alpha} \tau^0_{\gamma,\alpha} \tau^4_{\gamma,\alpha} \quad (3r_T r_V N_v) \quad (197)$$

$${}^1R_{a,i} \leftarrow \sum_{\gamma \in A} Y^2_{i,\gamma} \tau^5_{\gamma,a} \quad (2r_T N_o N_v) \quad (198)$$

Raw expression

$${}^1R_{a,i} \leftarrow \sum_{j \in O} \sum_{b \in V} \sum_{c \in V} {}^2T_{b,j,c,i} V_{a,c,j,b} \quad (199)$$

Factorized expression

$$\tau^0_{\gamma,\alpha} = \sum_{a \in V} W^2_{a,\alpha} Y^3_{a,\gamma} \quad (2r_T r_V N_v) \quad (200)$$

$$\tau^1_{\gamma,\alpha} = \sum_{i \in O} W^3_{i,\alpha} Y^2_{i,\gamma} \quad (2r_T r_V N_o) \quad (201)$$

$$\tau^2_{\gamma,\alpha} = \sum_{a \in V} W^4_{a,\alpha} Y^1_{a,\gamma} \quad (2r_T r_V N_v) \quad (202)$$

$$\tau^3_{\gamma,\alpha} = \sum_{\beta \in B} X_{\alpha,\beta} \tau^1_{\gamma,\beta} \tau^2_{\gamma,\beta} \quad (3r_T r_V^2) \quad (203)$$

$$\tau^4_{\gamma,\alpha} = \sum_{\delta \in A} Z_{\delta,\gamma} \tau^3_{\delta,\alpha} \quad (2r_T^2 r_V) \quad (204)$$

$$\tau^5_{\gamma,a} = \sum_{\alpha \in B} W^1_{a,\alpha} \tau^0_{\gamma,\alpha} \tau^4_{\gamma,\alpha} \quad (3r_T r_V N_v) \quad (205)$$

$${}^1R_{a,i} \leftarrow \sum_{\gamma \in A} Y^4_{i,\gamma} \tau^5_{\gamma,a} \quad (2r_T N_o N_v) \quad (206)$$

Raw expression

$${}^1R_{a,i} \leftarrow - \sum_{j \in O} \sum_{b \in V} \sum_{c \in V} \frac{1}{2} {}^2T_{b,i,c,j} V_{a,c,j,b} \quad (207)$$

Factorized expression

$$\tau^0_{\gamma,\alpha} = \sum_{a \in V} W^2_{a,\alpha} Y^1_{a,\gamma} \quad (2r_T r_V N_v) \quad (208)$$

$$\tau^1_{\gamma,\alpha} = \sum_{i \in O} W^3_{i,\alpha} Y^2_{i,\gamma} \quad (2r_T r_V N_o) \quad (209)$$

$$\tau^2_{\gamma,\alpha} = \sum_{a \in V} W^4_{a,\alpha} Y^3_{a,\gamma} \quad (2r_T r_V N_v) \quad (210)$$

$$\tau^3_{\gamma,\alpha} = \sum_{\delta \in A} \sum_{\beta \in B} X_{\alpha,\beta} Z_{\delta,\gamma} \tau^0_{\delta,\alpha} \tau^1_{\delta,\beta} \tau^2_{\gamma,\beta} \quad (5r_T^2 r_V^2) \quad (211)$$

$$\tau^4_{\gamma,a} = \sum_{\alpha \in B} W^1_{a,\alpha} \tau^3_{\gamma,\alpha} \quad (2r_T r_V N_v) \quad (212)$$

$${}^1R_{a,i} \leftarrow - \sum_{\gamma \in A} \frac{1}{2} Y^4_{i,\gamma} \tau^4_{\gamma,a} \quad (2r_T N_o N_v) \quad (213)$$

Raw expression

$${}^1R_{a,i} \leftarrow - \sum_{j \in O} \sum_{b \in V} \sum_{c \in V} \frac{1}{2} {}^2T_{b,j,c,i} V_{a,b,j,c} \quad (214)$$

Factorized expression

$$\tau^0_{\gamma,\alpha} = \sum_{a \in V} W^2_{a,\alpha} Y^3_{a,\gamma} \quad (2r_T r_V N_v) \quad (215)$$

$$\tau^1_{\gamma,\alpha} = \sum_{i \in O} W^3_{i,\alpha} Y^4_{i,\gamma} \quad (2r_T r_V N_o) \quad (216)$$

$$\tau^2_{\gamma,\alpha} = \sum_{a \in V} W^4_{a,\alpha} Y^1_{a,\gamma} \quad (2r_T r_V N_v) \quad (217)$$

$$\tau^3_{\gamma,\alpha} = \sum_{\delta \in A} \sum_{\beta \in B} X_{\alpha,\beta} Z_{\gamma,\delta} \tau^0_{\delta,\alpha} \tau^1_{\delta,\beta} \tau^2_{\gamma,\beta} \quad (5r_T^2 r_V^2) \quad (218)$$

$$\tau^4_{\gamma,a} = \sum_{\alpha \in B} W^1_{a,\alpha} \tau^3_{\gamma,\alpha} \quad (2r_T r_V N_v) \quad (219)$$

$${}^1R_{a,i} \leftarrow - \sum_{\gamma \in A} \frac{1}{2} Y^2_{i,\gamma} \tau^4_{\gamma,a} \quad (2r_T N_o N_v) \quad (220)$$

Raw expression

$${}^1R_{a,i} \leftarrow \sum_{j \in O} \sum_{b \in V} f_{j,b} {}^2T_{a,i,b,j} \quad (221)$$

Factorized expression

$$\tau^0_{\gamma,\alpha} = \sum_{i \in O} W^1_{i,\alpha} Y^4_{i,\gamma} \quad (2r_T r_V N_o) \quad (222)$$

$$\tau^1_{\gamma,\alpha} = \sum_{i \in O} W^3_{i,\alpha} Y^2_{i,\gamma} \quad (2r_T r_V N_o) \quad (223)$$

$$\tau^2_{\gamma,\alpha} = \sum_{a \in V} W^4_{a,\alpha} Y^3_{a,\gamma} \quad (2r_T r_V N_v) \quad (224)$$

$$\tau^3_{\gamma,\alpha} = \sum_{\delta \in A} \sum_{\beta \in B} X_{\alpha,\beta} Z_{\gamma,\delta} \tau^0_{\delta,\alpha} \tau^1_{\gamma,\beta} \tau^2_{\delta,\beta} \quad (5r_T^2 r_V^2) \quad (225)$$

$$\tau^4_{\gamma,i} = \sum_{\alpha \in B} W^2_{i,\alpha} \tau^3_{\gamma,\alpha} \quad (2r_T r_V N_o) \quad (226)$$

$${}^1R_{a,i} \leftarrow \sum_{\gamma \in A} \frac{1}{2} Y^1_{a,\gamma} \tau^4_{\gamma,i} \quad (2r_T N_o N_v) \quad (227)$$

Raw expression

$${}^1R_{a,i} \leftarrow \sum_{j \in O} \sum_{b \in V} f_{j,b} {}^2T_{b,j,a,i} \quad (228)$$

Factorized expression

$$\tau^0_{\gamma,\alpha} = \sum_{i \in O} W^1_{i,\alpha} Y^2_{i,\gamma} \quad (2r_T r_V N_o) \quad (229)$$

$${}^1R_{a,i} \leftarrow - \sum_{j \in O} \sum_{b \in V} \frac{1}{2} f_{j,b} {}^2T_{b,i,a,j} \quad (243)$$

$$\tau^1_{\gamma,\alpha} = \sum_{i \in O} W^3_{i,\alpha} Y^4_{i,\gamma} \quad (2r_T r_V N_o) \quad (230)$$

Factorized expression

$$\tau^2_{\gamma,\alpha} = \sum_{a \in V} W^4_{a,\alpha} Y^1_{a,\gamma} \quad (2r_T r_V N_v) \quad (231)$$

$$\tau^0_{\gamma,\alpha} = \sum_{i \in O} W^1_{i,\alpha} Y^4_{i,\gamma} \quad (2r_T r_V N_o) \quad (244)$$

$$\tau^3_{\gamma,\alpha} = \sum_{\delta \in A} \sum_{\beta \in B} X_{\alpha,\beta} Z_{\delta,\gamma} \tau^0_{\delta,\alpha} \tau^1_{\gamma,\beta} \tau^2_{\delta,\beta} \quad (5r_T^2 r_V^2) \quad (232)$$

$$\tau^1_{\gamma,\alpha} = \sum_{i \in O} W^3_{i,\alpha} Y^2_{i,\gamma} \quad (2r_T r_V N_o) \quad (245)$$

$$\tau^4_{\gamma,i} = \sum_{\alpha \in B} W^2_{i,\alpha} \tau^3_{\gamma,\alpha} \quad (2r_T r_V N_o) \quad (233)$$

$$\tau^2_{\gamma,\alpha} = \sum_{a \in V} W^4_{a,\alpha} Y^1_{a,\gamma} \quad (2r_T r_V N_v) \quad (246)$$

$${}^1R_{a,i} \leftarrow \sum_{\gamma \in A} \frac{1}{2} Y^3_{a,\gamma} \tau^4_{\gamma,i} \quad (2r_T N_o N_v) \quad (234)$$

$$\tau^3_{\gamma,\alpha} = \sum_{\beta \in B} X_{\alpha,\beta} \tau^1_{\gamma,\beta} \tau^2_{\gamma,\beta} \quad (3r_T r_V^2) \quad (247)$$

Raw expression

$$\tau^4_{\gamma,\alpha} = \sum_{\delta \in A} Z_{\delta,\gamma} \tau^3_{\delta,\alpha} \quad (2r_T^2 r_V) \quad (248)$$

$${}^1R_{a,i} \leftarrow - \sum_{j \in O} \sum_{b \in V} \frac{1}{2} f_{j,b} {}^2T_{a,j,b,i} \quad (235)$$

$$\tau^5_{\gamma,i} = \sum_{\alpha \in B} W^2_{i,\alpha} \tau^0_{\gamma,\alpha} \tau^4_{\gamma,\alpha} \quad (3r_T r_V N_o) \quad (249)$$

Factorized expression

$$\tau^0_{\gamma,\alpha} = \sum_{i \in O} W^1_{i,\alpha} Y^2_{i,\gamma} \quad (2r_T r_V N_o) \quad (236)$$

$${}^1R_{a,i} \leftarrow - \sum_{\gamma \in A} Y^3_{a,\gamma} \tau^5_{\gamma,i} \quad (2r_T N_o N_v) \quad (250)$$

Raw expression

$$\tau^1_{\gamma,\alpha} = \sum_{i \in O} W^3_{i,\alpha} Y^4_{i,\gamma} \quad (2r_T r_V N_o) \quad (237)$$

$${}^1R_{a,i} \leftarrow \sum_{j \in O} \sum_{k \in O} \sum_{b \in V} \frac{1}{2} {}^2T_{a,j,b,k} V_{k,i,j,b} \quad (251)$$

Factorized expression

$$\tau^2_{\gamma,\alpha} = \sum_{a \in V} W^4_{a,\alpha} Y^3_{a,\gamma} \quad (2r_T r_V N_v) \quad (238)$$

$$\tau^0_{\gamma,i} = \sum_{a \in V} Y^3_{a,\gamma} f_{i,a} \quad (2r_T N_o N_v) \quad (252)$$

$$\tau^3_{\gamma,\alpha} = \sum_{\beta \in B} X_{\alpha,\beta} \tau^1_{\gamma,\beta} \tau^2_{\gamma,\beta} \quad (3r_T r_V^2) \quad (239)$$

$$\tau^1_{\gamma} = \sum_{i \in O} Y^4_{i,\gamma} \tau^0_{\gamma,i} \quad (2r_T N_o) \quad (253)$$

$$\tau^4_{\gamma,\alpha} = \sum_{\delta \in A} Z_{\gamma,\delta} \tau^3_{\delta,\alpha} \quad (2r_T^2 r_V) \quad (240)$$

$$\tau^2_{\gamma} = \sum_{\delta \in A} \tau^1_p Z_{\gamma,\delta} \quad (2r_T^2) \quad (254)$$

$$\tau^5_{\gamma,i} = \sum_{\alpha \in B} W^2_{i,\alpha} \tau^0_{\gamma,\alpha} \tau^4_{\gamma,\alpha} \quad (3r_T r_V N_o) \quad (241)$$

$${}^1R_{a,i} \leftarrow \sum_{\gamma \in A} \tau^2_{\gamma} Y^1_{a,\gamma} Y^2_{i,\gamma} \quad (3r_T N_o N_v) \quad (255)$$

$${}^1R_{a,i} \leftarrow - \sum_{\gamma \in A} Y^1_{a,\gamma} \tau^5_{\gamma,i} \quad (2r_T N_o N_v) \quad (242)$$

Raw expression

$${}^1R_{a,i} \leftarrow \sum_{j \in O} \sum_{k \in O} \sum_{b \in V} \frac{1}{2} {}^2T_{b,j,a,k} V_{j,i,k,b} \quad (256)$$

Raw expression

Factorized expression

$$\tau^0_{\gamma,i} = \sum_{a \in V} Y^1_{a,\gamma} f_{i,a} \quad (2r_T N_o N_v) \quad (257)$$

$$\tau^1_{\gamma} = \sum_{i \in O} Y^2_{i,\gamma} \tau^0_{\gamma,i} \quad (2r_T N_o) \quad (258)$$

$$\tau^2_{\gamma} = \sum_{\delta \in A} \tau^1_{\gamma} Z_{\delta,\gamma} \quad (2r_T^2) \quad (259)$$

$${}^1R_{a,i} \leftarrow \sum_{\gamma \in A} \tau^2_{\gamma} Y^3_{a,\gamma} Y^4_{i,\gamma} \quad (3r_T N_o N_v) \quad (260)$$

Raw expression

$${}^1R_{a,i} \leftarrow - \sum_{j \in O} \sum_{k \in O} \sum_{b \in V} {}^2T_{a,j,b,k} V_{j,i,k,b} \quad (261)$$

Factorized expression

$$\tau^0_{\gamma,i} = \sum_{a \in V} Y^3_{a,\gamma} f_{i,a} \quad (2r_T N_o N_v) \quad (262)$$

$$\tau^1_{\gamma,\delta} = \sum_{i \in O} Y^2_{i,\gamma} \tau^0_{\delta,i} \quad (2r_T^2 N_o) \quad (263)$$

$$\tau^2_{\gamma,i} = \sum_{\delta \in A} Z_{\gamma,\delta} Y^4_{i,\delta} \tau^1_{\gamma,\delta} \quad (3r_T^2 N_o) \quad (264)$$

$${}^1R_{a,i} \leftarrow - \sum_{\gamma \in A} \frac{1}{2} Y^1_{a,\gamma} \tau^2_{\gamma,i} \quad (2r_T N_o N_v) \quad (265)$$

Raw expression

$${}^1R_{a,i} \leftarrow - \sum_{j \in O} \sum_{k \in O} \sum_{b \in V} {}^2T_{b,j,a,k} V_{k,i,j,b} \quad (266)$$

Factorized expression

$$\tau^0_{\gamma,i} = \sum_{a \in V} Y^1_{a,\gamma} f_{i,a} \quad (2r_T N_o N_v) \quad (267)$$

$$\tau^1_{\gamma,\delta} = \sum_{i \in O} Y^4_{i,\delta} \tau^0_{\gamma,i} \quad (2r_T^2 N_o) \quad (268)$$

$$\tau^2_{\gamma,a} = \sum_{\delta \in A} Z_{\gamma,\delta} Y^3_{a,\delta} \tau^1_{\gamma,\delta} \quad (3r_T^2 N_v) \quad (269)$$

$${}^1R_{a,i} \leftarrow - \sum_{\gamma \in A} \frac{1}{2} Y^2_{i,\gamma} \tau^2_{\gamma,a} \quad (2r_T N_o N_v) \quad (270)$$

**E. Contributions from  $(H^1 T^1 T^1 T)_c$** 

Raw expression

$${}^1R_{a,i} \leftarrow \sum_{j \in O} \sum_{k \in O} \sum_{b \in V} \sum_{c \in V} {}^1T_{a,j} {}^1T_{b,i} {}^1T_{c,k} V_{j,c,k,b} \quad (271)$$

Factorized expression

$$\tau^0_{\alpha,i} = \sum_{a \in V} {}^1T_{a,i} W^2_{a,\alpha} \quad (2r_V N_o N_v) \quad (272)$$

$$\tau^1_{\alpha,\beta} = \sum_{i \in O} W^3_{i,\beta} \tau^0_{\alpha,i} \quad (2r_V^2 N_o) \quad (273)$$

$$\tau^2_{\alpha,a} = \sum_{\beta \in B} X_{\alpha,\beta} W^4_{a,\beta} \tau^1_{\alpha,\beta} \quad (3r_V^2 N_v) \quad (274)$$

$$\tau^3_{i,a} = \sum_{\alpha \in B} W^1_{i,\alpha} \tau^2_{\alpha,a} \quad (2r_V N_o N_v) \quad (275)$$

$$\tau^4_{i,j} = \sum_{a \in V} {}^1T_{a,i} \tau^3_{j,a} \quad (2N_o^2 N_v) \quad (276)$$

$${}^1R_{a,i} \leftarrow \sum_{j \in O} {}^1T_{a,j} \tau^4_{i,j} \quad (2N_o^2 N_v) \quad (277)$$

Raw expression

$${}^1R_{a,i} \leftarrow - \sum_{j \in O} \sum_{k \in O} \sum_{b \in V} \sum_{c \in V} 2 {}^1T_{a,j} {}^1T_{b,i} {}^1T_{c,k} V_{j,b,k,c} \quad (278)$$

Factorized expression

$$\tau^0_{\alpha,i} = \sum_{a \in V} {}^1T_{a,i} W^4_{a,\alpha} \quad (2r_V N_o N_v) \quad (279)$$

$$\tau^1_{\alpha} = \sum_{i \in O} W^3_{i,\alpha} \tau^0_{\alpha,i} \quad (2r_V N_o) \quad (280)$$

$$\tau^2_{\alpha} = \sum_{\beta \in B} \tau^1_{\beta} X_{\alpha,\beta} \quad (2r_V^2) \quad (281)$$

$$\tau^3_{i,a} = \sum_{\alpha \in B} \tau^2_{\alpha} W^1_{i,\alpha} W^2_{a,\alpha} \quad (3r_V N_o N_v) \quad (282)$$

$$\tau^4_{i,j} = \sum_{a \in V} {}^1T_{a,i} \tau^3_{j,a} \quad (2N_o^2 N_v) \quad (283)$$

$${}^1R_{a,i} \leftarrow - \sum_{j \in O} 2 {}^1T_{a,j} \tau^4_{i,j} \quad (2N_o^2 N_v) \quad (284)$$

### F. Contributions from $(H^1 T^2 T)_c$

Raw expression

$${}^1R_{a,i} \leftarrow \sum_{j \in O} \sum_{k \in O} \sum_{b \in V} \sum_{c \in V} \frac{1}{2} {}^1T_{a,j} {}^2T_{b,i,c,k} V_{j,c,k,b} \quad (285)$$

Factorized expression

$$\tau^0_{\gamma,\alpha} = \sum_{a \in V} W^2_{a,\alpha} Y^1_{a,\gamma} \quad (2r_T r_V N_v) \quad (286)$$

$$\tau^1_{\gamma,\alpha} = \sum_{i \in O} W^3_{i,\alpha} Y^2_{i,\gamma} \quad (2r_T r_V N_o) \quad (287)$$

$$\tau^2_{\gamma,\alpha} = \sum_{a \in V} W^4_{a,\alpha} Y^3_{a,\gamma} \quad (2r_T r_V N_v) \quad (288)$$

$$\tau^3_{\gamma,\alpha} = \sum_{\delta \in A} \sum_{\beta \in B} X_{\alpha,\beta} Z_{\delta,\gamma} \tau^0_{\delta,\alpha} \tau^1_{\delta,\beta} \tau^2_{\gamma,\beta} \quad (5r_T^2 r_V^2) \quad (289)$$

$$\tau^4_{\gamma,i} = \sum_{\alpha \in B} W^1_{i,\alpha} \tau^3_{\gamma,\alpha} \quad (2r_T r_V N_o) \quad (290)$$

$$\tau^5_{i,j} = \sum_{\gamma \in A} Y^4_{j,\gamma} \tau^4_{\gamma,i} \quad (2r_T N_o^2) \quad (291)$$

$${}^1R_{a,i} \leftarrow \sum_{j \in O} \frac{1}{2} {}^1T_{a,j} \tau^5_{j,i} \quad (2N_o^2 N_v) \quad (292)$$

Raw expression

$${}^1R_{a,i} \leftarrow \sum_{j \in O} \sum_{k \in O} \sum_{b \in V} \sum_{c \in V} \frac{1}{2} {}^1T_{a,j} {}^2T_{b,k,c,i} V_{j,b,k,c} \quad (293)$$

Factorized expression

$$\tau^0_{\gamma,\alpha} = \sum_{a \in V} W^2_{a,\alpha} Y^3_{a,\gamma} \quad (2r_T r_V N_v) \quad (294)$$

$$\tau^1_{\gamma,\alpha} = \sum_{i \in O} W^3_{i,\alpha} Y^4_{i,\gamma} \quad (2r_T r_V N_o) \quad (295)$$

$$\tau^2_{\gamma,\alpha} = \sum_{a \in V} W^4_{a,\alpha} Y^1_{a,\gamma} \quad (2r_T r_V N_v) \quad (296)$$

$$\tau^3_{\gamma,\alpha} = \sum_{\delta \in A} \sum_{\beta \in B} X_{\alpha,\beta} Z_{\gamma,\delta} \tau^0_{\delta,\alpha} \tau^1_{\delta,\beta} \tau^2_{\gamma,\beta} \quad (5r_T^2 r_V^2) \quad (297)$$

$$\tau^4_{\gamma,i} = \sum_{\alpha \in B} W^1_{i,\alpha} \tau^3_{\gamma,\alpha} \quad (2r_T r_V N_o) \quad (298)$$

$$\tau^5_{i,j} = \sum_{\gamma \in A} Y^2_{j,\gamma} \tau^4_{\gamma,i} \quad (2r_T N_o^2) \quad (299)$$

$${}^1R_{a,i} \leftarrow \sum_{j \in O} \frac{1}{2} {}^1T_{a,j} \tau^5_{j,i} \quad (2N_o^2 N_v) \quad (300)$$

Raw expression

$${}^1R_{a,i} \leftarrow \sum_{j \in O} \sum_{k \in O} \sum_{b \in V} \sum_{c \in V} \frac{1}{2} {}^1T_{b,i} {}^2T_{a,j,c,k} V_{j,c,k,b} \quad (301)$$

Factorized expression

$$\tau^0_{\gamma,\alpha} = \sum_{i \in O} W^1_{i,\alpha} Y^2_{i,\gamma} \quad (2r_T r_V N_o) \quad (302)$$

$$\tau^1_{\gamma,\alpha} = \sum_{i \in O} W^3_{i,\alpha} Y^4_{i,\gamma} \quad (2r_T r_V N_o) \quad (303)$$

$$\tau^2_{\gamma,\alpha} = \sum_{a \in V} W^4_{a,\alpha} Y^1_{a,\gamma} \quad (2r_T r_V N_v) \quad (304)$$

$$\tau^3_{\gamma,\alpha} = \sum_{\delta \in A} \sum_{\beta \in B} X_{\alpha,\beta} Z_{\delta,\gamma} \tau^0_{\delta,\alpha} \tau^1_{\gamma,\beta} \tau^2_{\delta,\beta} \quad (5r_T^2 r_V^2) \quad (305)$$

$$\tau^4_{\gamma,a} = \sum_{\alpha \in B} W^2_{a,\alpha} \tau^3_{\gamma,\alpha} \quad (2r_T r_V N_v) \quad (306)$$

$$\tau^5_{a,b} = \sum_{\gamma \in A} Y^3_{b,\gamma} \tau^4_{\gamma,a} \quad (2r_T N_v^2) \quad (307)$$

$${}^1R_{a,i} \leftarrow \sum_{b \in V} \frac{1}{2} {}^1T_{b,i} \tau^5_{b,a} \quad (2N_o N_v^2) \quad (308)$$

Raw expression

$${}^1R_{a,i} \leftarrow \sum_{j \in O} \sum_{k \in O} \sum_{b \in V} \sum_{c \in V} \frac{1}{2} {}^1T_{b,i} {}^2T_{c,j,a,k} V_{j,b,k,c} \quad (309)$$

Factorized expression

$$\tau^0_{\gamma,\alpha} = \sum_{i \in O} W^1_{i,\alpha} Y^2_{i,\gamma} \quad (2r_T r_V N_o) \quad (310)$$

$$\tau^1_{\gamma,\alpha} = \sum_{a \in V} W^2_{a,\alpha} Y^3_{a,\gamma} \quad (2r_T r_V N_v) \quad (311)$$

$$\tau^2_{\gamma,\alpha} = \sum_{i \in O} W^3_{i,\alpha} Y^4_{i,\gamma} \quad (2r_T r_V N_o) \quad (312)$$

$$\tau^3_{\gamma,\alpha} = \sum_{\delta \in A} \sum_{\beta \in B} X_{\beta,\alpha} Z_{\gamma,\delta} \tau^0_{\gamma,\beta} \tau^1_{\delta,\beta} \tau^2_{\delta,\alpha} \quad (5r_T^2 r_V^2) \quad (313)$$

$$\tau^4_{\gamma,a} = \sum_{\alpha \in B} W^4_{a,\alpha} \tau^3_{\gamma,\alpha} \quad (2r_T r_V N_v) \quad (314)$$

$$\tau^5_{a,b} = \sum_{\gamma \in A} Y^1_{b,\gamma} \tau^4_{\gamma,a} \quad (2r_T N_v^2) \quad (315)$$

$${}^1R_{a,i} \leftarrow \sum_{b \in V} \frac{1}{2} {}^1T_{b,i} \tau^5_{b,a} \quad (2N_o N_v^2) \quad (316)$$

Raw expression

$${}^1R_{a,i} \leftarrow \sum_{j \in O} \sum_{k \in O} \sum_{b \in V} \sum_{c \in V} \frac{1}{2} {}^1T_{b,j} {}^2T_{a,k,c,i} V_{j,c,k,b} \quad (317)$$

Factorized expression

$$\tau^0_{\alpha,i} = \sum_{a \in V} {}^1T_{a,i} W^4_{a,\alpha} \quad (2r_V N_o N_v) \quad (318)$$

$$\tau^1_{\alpha,\beta} = \sum_{i \in O} W^1_{i,\alpha} \tau^0_{\beta,i} \quad (2r_V^2 N_o) \quad (319)$$

$$\tau^2_{\alpha,i} = \sum_{\beta \in B} X_{\alpha,\beta} W^3_{i,\beta} \tau^1_{\alpha,\beta} \quad (3r_V^2 N_o) \quad (320)$$

$$\tau^3_{i,a} = \sum_{\alpha \in B} W^2_{a,\alpha} \tau^2_{\alpha,i} \quad (2r_V N_o N_v) \quad (321)$$

$$\tau^4_{\gamma,i} = \sum_{a \in V} Y^3_{a,\gamma} \tau^3_{i,a} \quad (2r_T N_o N_v) \quad (322)$$

$$\tau^5_{\gamma,\delta} = \sum_{i \in O} Y^2_{i,\gamma} \tau^4_{\delta,i} \quad (2r_T^2 N_o) \quad (323)$$

$$\tau^6_{\gamma,i} = \sum_{\delta \in A} Z_{\gamma,\delta} Y^4_{i,\delta} \tau^5_{\gamma,\delta} \quad (3r_T^2 N_o) \quad (324)$$

$${}^1R_{a,i} \leftarrow \sum_{\gamma \in A} \frac{1}{2} Y^1_{a,\gamma} \tau^6_{\gamma,i} \quad (2r_T N_o N_v) \quad (325)$$

Raw expression

$${}^1R_{a,i} \leftarrow \sum_{j \in O} \sum_{k \in O} \sum_{b \in V} \sum_{c \in V} \frac{1}{2} {}^1T_{b,j} {}^2T_{c,i,a,k} V_{j,c,k,b} \quad (326)$$

Factorized expression

$$\tau^0_{\alpha,i} = \sum_{a \in V} {}^1T_{a,i} W^4_{a,\alpha} \quad (2r_V N_o N_v) \quad (327)$$

$$\tau^1_{\alpha,\beta} = \sum_{i \in O} W^1_{i,\alpha} \tau^0_{\beta,i} \quad (2r_V^2 N_o) \quad (328)$$

$$\tau^2_{\alpha,i} = \sum_{\beta \in B} X_{\alpha,\beta} W^3_{i,\beta} \tau^1_{\alpha,\beta} \quad (3r_V^2 N_o) \quad (329)$$

$$\tau^3_{i,a} = \sum_{\alpha \in B} W^2_{a,\alpha} \tau^2_{\alpha,i} \quad (2r_V N_o N_v) \quad (330)$$

$$\tau^4_{\gamma,i} = \sum_{a \in V} Y^1_{a,\gamma} \tau^3_{i,a} \quad (2r_T N_o N_v) \quad (331)$$

$$\tau^5_{\gamma,\delta} = \sum_{i \in O} Y^4_{i,\delta} \tau^4_{\gamma,i} \quad (2r_T^2 N_o) \quad (332)$$

$$\tau^6_{\gamma,a} = \sum_{\delta \in A} Z_{\gamma,\delta} Y^3_{a,\delta} \tau^5_{\gamma,\delta} \quad (3r_T^2 N_v) \quad (333)$$

$${}^1R_{a,i} \leftarrow \sum_{\gamma \in A} \frac{1}{2} Y^2_{i,\gamma} \tau^6_{\gamma,a} \quad (2r_T N_o N_v) \quad (334)$$

Raw expression

$${}^1R_{a,i} \leftarrow - \sum_{j \in O} \sum_{k \in O} \sum_{b \in V} \sum_{c \in V} {}^1T_{a,j} {}^2T_{b,i,c,k} V_{j,b,k,c} \quad (335)$$

Factorized expression

$$\tau^0_{\gamma,\alpha} = \sum_{a \in V} W^2_{a,\alpha} Y^1_{a,\gamma} \quad (2r_T r_V N_v) \quad (336)$$

$$\tau^1_{\gamma,\alpha} = \sum_{i \in O} W^3_{i,\alpha} Y^4_{i,\gamma} \quad (2r_T r_V N_o) \quad (337)$$

$$\tau^2_{\gamma,\alpha} = \sum_{a \in V} W^4_{a,\alpha} Y^3_{a,\gamma} \quad (2r_T r_V N_v) \quad (338)$$

$$\tau^3_{\gamma,\alpha} = \sum_{\beta \in B} X_{\alpha,\beta} \tau^1_{\gamma,\beta} \tau^2_{\gamma,\beta} \quad (3r_T r_V^2) \quad (339)$$

$$\tau^4_{\gamma,\alpha} = \sum_{\delta \in A} Z_{\gamma,\delta} \tau^3_{\delta,\alpha} \quad (2r_T^2 r_V) \quad (340)$$

$$\tau^5_{\gamma,i} = \sum_{\alpha \in B} W^1_{i,\alpha} \tau^0_{\gamma,\alpha} \tau^4_{\gamma,\alpha} \quad (3r_T r_V N_o) \quad (341)$$

$$\tau^6_{i,j} = \sum_{\gamma \in A} Y^2_{j,\gamma} \tau^5_{\gamma,i} \quad (2r_T N_o^2) \quad (342)$$

$${}^1R_{a,i} \leftarrow - \sum_{j \in O} {}^1T_{a,j} \tau^6_{j,i} \quad (2N_o^2 N_v) \quad (343)$$

Raw expression

$${}^1R_{a,i} \leftarrow - \sum_{j \in O} \sum_{k \in O} \sum_{b \in V} \sum_{c \in V} {}^1T_{a,j} {}^2T_{b,k,c,i} V_{j,c,k,b} \quad (344)$$

Factorized expression

$$\tau^0_{\gamma,\alpha} = \sum_{a \in V} W^2_{a,\alpha} Y^3_{a,\gamma} \quad (2r_T r_V N_v) \quad (345)$$

$$\tau^1_{\gamma,\alpha} = \sum_{i \in O} W^3_{i,\alpha} Y^2_{i,\gamma} \quad (2r_T r_V N_o) \quad (346)$$

$$\tau^2_{\gamma,\alpha} = \sum_{a \in V} W^4_{a,\alpha} Y^1_{a,\gamma} \quad (2r_T r_V N_v) \quad (347)$$

$$\tau^3_{\gamma,\alpha} = \sum_{\beta \in B} X_{\alpha,\beta} \tau^1_{\gamma,\beta} \tau^2_{\gamma,\beta} \quad (3r_T r_V^2) \quad (348)$$

$$\tau^4_{\gamma,\alpha} = \sum_{\delta \in A} Z_{\gamma,\delta} \tau^3_{\delta,\alpha} \quad (2r_T^2 r_V) \quad (349)$$

$$\tau^5_{\gamma,i} = \sum_{\alpha \in B} W^1_{i,\alpha} \tau^0_{\gamma,\alpha} \tau^4_{\gamma,\alpha} \quad (3r_T r_V N_o) \quad (350)$$

$$\tau^6_{i,j} = \sum_{\gamma \in A} Y^4_{j,\gamma} \tau^5_{\gamma,i} \quad (2r_T N_o^2) \quad (351)$$

$${}^1R_{a,i} \leftarrow - \sum_{j \in O} {}^1T_{a,j} \tau^6_{j,i} \quad (2N_o^2 N_v) \quad (352)$$

Raw expression

$${}^1R_{a,i} \leftarrow - \sum_{j \in O} \sum_{k \in O} \sum_{b \in V} \sum_{c \in V} {}^1T_{b,i} {}^2T_{a,j,c,k} V_{j,b,k,c} \quad (353)$$

Factorized expression

$$\tau^0_{\gamma,\alpha} = \sum_{i \in O} W^1_{i,\alpha} Y^2_{i,\gamma} \quad (2r_T r_V N_o) \quad (354)$$

$$\tau^1_{\gamma,\alpha} = \sum_{i \in O} W^3_{i,\alpha} Y^4_{i,\gamma} \quad (2r_T r_V N_o) \quad (355)$$

$$\tau^2_{\gamma,\alpha} = \sum_{a \in V} W^4_{a,\alpha} Y^3_{a,\gamma} \quad (2r_T r_V N_v) \quad (356)$$

$$\tau^3_{\gamma,\alpha} = \sum_{\beta \in B} X_{\alpha,\beta} \tau^1_{\gamma,\beta} \tau^2_{\gamma,\beta} \quad (3r_T r_V^2) \quad (357)$$

$$\tau^4_{\gamma,\alpha} = \sum_{\delta \in A} Z_{\gamma,\delta} \tau^3_{\delta,\alpha} \quad (2r_T^2 r_V) \quad (358)$$

$$\tau^5_{\gamma,a} = \sum_{\alpha \in B} W^2_{a,\alpha} \tau^0_{\gamma,\alpha} \tau^4_{\gamma,\alpha} \quad (3r_T r_V N_v) \quad (359)$$

$$\tau^6_{a,b} = \sum_{\gamma \in A} Y^1_{b,\gamma} \tau^5_{\gamma,a} \quad (2r_T N_v^2) \quad (360)$$

$${}^1R_{a,i} \leftarrow - \sum_{b \in V} {}^1T_{b,i} \tau^6_{b,a} \quad (2N_o N_v^2) \quad (361)$$

Raw expression

$${}^1R_{a,i} \leftarrow - \sum_{j \in O} \sum_{k \in O} \sum_{b \in V} \sum_{c \in V} {}^1T_{b,i} {}^2T_{c,j,a,k} V_{j,c,k,b} \quad (362)$$

Factorized expression

$$\tau^0_{\gamma,\alpha} = \sum_{i \in O} W^1_{i,\alpha} Y^2_{i,\gamma} \quad (2r_T r_V N_o) \quad (363)$$

$$\tau^1_{\gamma,\alpha} = \sum_{a \in V} W^2_{a,\alpha} Y^1_{a,\gamma} \quad (2r_T r_V N_v) \quad (364)$$

$$\tau^2_{\gamma,\alpha} = \sum_{\beta \in B} X_{\beta,\alpha} \tau^0_{\gamma,\beta} \tau^1_{\gamma,\beta} \quad (3r_T r_V^2) \quad (365)$$

$${}^1R_{a,i} \leftarrow - \sum_{j \in O} \sum_{k \in O} \sum_{b \in V} \sum_{c \in V} {}^1T_{b,j} {}^2T_{a,k,c,i} V_{j,b,k,c} \quad (380)$$

Factorized expression

$$\tau^0_{\alpha,i} = \sum_{a \in V} {}^1T_{a,i} W^2_{a,\alpha} \quad (2r_V N_o N_v) \quad (381)$$

$$\tau^1_{\alpha} = \sum_{i \in O} W^1_{i,\alpha} \tau^0_{\alpha,i} \quad (2r_V N_o) \quad (382)$$

$$\tau^2_{\alpha} = \sum_{\beta \in B} \tau^1_{\beta} X_{\beta,\alpha} \quad (2r_V^2) \quad (383)$$

$$\tau^3_{i,a} = \sum_{\alpha \in B} \tau^2_{\alpha} W^3_{i,\alpha} W^4_{a,\alpha} \quad (3r_V N_o N_v) \quad (384)$$

$$\tau^4_{\gamma,i} = \sum_{a \in V} Y^1_{a,\gamma} \tau^3_{i,a} \quad (2r_T N_o N_v) \quad (385)$$

$$\tau^5_{\gamma,\delta} = \sum_{i \in O} Y^4_{i,\delta} \tau^4_{\gamma,i} \quad (2r_T^2 N_o) \quad (386)$$

$$\tau^6_{\gamma,a} = \sum_{\delta \in A} Z_{\gamma,\delta} Y^3_{a,\delta} \tau^5_{\gamma,\delta} \quad (3r_T^2 N_v) \quad (387)$$

$${}^1R_{a,i} \leftarrow - \sum_{\gamma \in A} Y^2_{i,\gamma} \tau^6_{\gamma,a} \quad (2r_T N_o N_v) \quad (388)$$

Raw expression

$${}^1R_{a,i} \leftarrow - \sum_{j \in O} \sum_{k \in O} \sum_{b \in V} \sum_{c \in V} {}^1T_{b,j} {}^2T_{c,i,a,k} V_{j,b,k,c} \quad (389)$$

Factorized expression

$$\tau^0_{\alpha,i} = \sum_{a \in V} {}^1T_{a,i} W^4_{a,\alpha} \quad (2r_V N_o N_v) \quad (390)$$

$$\tau^1_{\alpha,\beta} = \sum_{i \in O} W^1_{i,\alpha} \tau^0_{\beta,i} \quad (2r_V^2 N_o) \quad (391)$$

$$\tau^2_{\alpha,i} = \sum_{\beta \in B} X_{\alpha,\beta} W^3_{i,\beta} \tau^1_{\alpha,\beta} \quad (3r_V^2 N_o) \quad (392)$$

$$\tau^3_{i,a} = \sum_{\alpha \in B} W^2_{a,\alpha} \tau^2_{\alpha,i} \quad (2r_V N_o N_v) \quad (393)$$

$$\tau^3_{\gamma,\alpha} = \sum_{\delta \in A} Z_{\delta,\gamma} \tau^2_{\delta,\alpha} \quad (2r_T^2 r_V) \quad (366)$$

$$\tau^4_{\gamma,\alpha} = \sum_{i \in O} W^3_{i,\alpha} Y^4_{i,\gamma} \quad (2r_T r_V N_o) \quad (367)$$

$$\tau^5_{\gamma,a} = \sum_{\alpha \in B} W^4_{a,\alpha} \tau^3_{\gamma,\alpha} \tau^4_{\gamma,\alpha} \quad (3r_T r_V N_v) \quad (368)$$

$$\tau^6_{a,b} = \sum_{\gamma \in A} Y^3_{b,\gamma} \tau^5_{\gamma,a} \quad (2r_T N_v^2) \quad (369)$$

$${}^1R_{a,i} \leftarrow - \sum_{b \in V} {}^1T_{b,i} \tau^6_{b,a} \quad (2N_o N_v^2) \quad (370)$$

Raw expression

$${}^1R_{a,i} \leftarrow - \sum_{j \in O} \sum_{k \in O} \sum_{b \in V} \sum_{c \in V} {}^1T_{b,j} {}^2T_{a,i,c,k} V_{j,b,k,b} \quad (371)$$

Factorized expression

$$\tau^0_{\alpha,i} = \sum_{a \in V} {}^1T_{a,i} W^2_{a,\alpha} \quad (2r_V N_o N_v) \quad (372)$$

$$\tau^1_{\alpha} = \sum_{i \in O} W^1_{i,\alpha} \tau^0_{\alpha,i} \quad (2r_V N_o) \quad (373)$$

$$\tau^2_{\alpha} = \sum_{\beta \in B} \tau^1_{\beta} X_{\beta,\alpha} \quad (2r_V^2) \quad (374)$$

$$\tau^3_{i,a} = \sum_{\alpha \in B} \tau^2_{\alpha} W^3_{i,\alpha} W^4_{a,\alpha} \quad (3r_V N_o N_v) \quad (375)$$

$$\tau^4_{\gamma,i} = \sum_{a \in V} Y^3_{a,\gamma} \tau^3_{i,a} \quad (2r_T N_o N_v) \quad (376)$$

$$\tau^5_{\gamma,\delta} = \sum_{i \in O} Y^2_{i,\gamma} \tau^4_{\delta,i} \quad (2r_T^2 N_o) \quad (377)$$

$$\tau^6_{\gamma,i} = \sum_{\delta \in A} Z_{\gamma,\delta} Y^4_{i,\delta} \tau^5_{\gamma,\delta} \quad (3r_T^2 N_o) \quad (378)$$

$${}^1R_{a,i} \leftarrow - \sum_{\gamma \in A} Y^1_{a,\gamma} \tau^6_{\gamma,i} \quad (2r_T N_o N_v) \quad (379)$$

Raw expression



Factorized expression

$$\tau^4_{\gamma,i} = \sum_{a \in V} Y^3_{a,\gamma} \tau^3_{i,a} \quad (2r_T N_o N_v) \quad (394)$$

$$\tau^5_{\gamma} = \sum_{i \in O} Y^4_{i,\gamma} \tau^4_{\gamma,i} \quad (2r_T N_o) \quad (395)$$

$$\tau^6_{\gamma} = \sum_{\delta \in A} \tau^5_p Z_{\gamma,\delta} \quad (2r_T^2) \quad (396)$$

$${}^1R_{a,i} \leftarrow - \sum_{\gamma \in A} \tau^6_{\gamma} Y^1_{a,\gamma} Y^2_{i,\gamma} \quad (3r_T N_o N_v) \quad (397)$$

Raw expression

$${}^1R_{a,i} \leftarrow - \sum_{j \in O} \sum_{k \in O} \sum_{b \in V} \sum_{c \in V} {}^1T_{b,j} {}^2T_{c,k,a,i} V_{j,c,k,b} \quad (398)$$

Factorized expression

$$\tau^0_{\alpha,i} = \sum_{a \in V} {}^1T_{a,i} W^4_{a,\alpha} \quad (2r_V N_o N_v) \quad (399)$$

$$\tau^1_{\alpha,\beta} = \sum_{i \in O} W^1_{i,\alpha} \tau^0_{\beta,i} \quad (2r_V^2 N_o) \quad (400)$$

$$\tau^2_{\alpha,i} = \sum_{\beta \in B} X_{\alpha,\beta} W^3_{i,\beta} \tau^1_{\alpha,\beta} \quad (3r_V^2 N_o) \quad (401)$$

$$\tau^3_{i,a} = \sum_{\alpha \in B} W^2_{a,\alpha} \tau^2_{\alpha,i} \quad (2r_V N_o N_v) \quad (402)$$

$$\tau^4_{\gamma,i} = \sum_{a \in V} Y^1_{a,\gamma} \tau^3_{i,a} \quad (2r_T N_o N_v) \quad (403)$$

$$\tau^5_{\gamma} = \sum_{i \in O} Y^2_{i,\gamma} \tau^4_{\gamma,i} \quad (2r_T N_o) \quad (404)$$

$$\tau^6_{\gamma} = \sum_{\delta \in A} \tau^5_p Z_{\delta,\gamma} \quad (2r_T^2) \quad (405)$$

$${}^1R_{a,i} \leftarrow - \sum_{\gamma \in A} \tau^6_{\gamma} Y^3_{a,\gamma} Y^4_{i,\gamma} \quad (3r_T N_o N_v) \quad (406)$$

Raw expression

$${}^1R_{a,i} \leftarrow \sum_{j \in O} \sum_{k \in O} \sum_{b \in V} \sum_{c \in V} 2 {}^1T_{b,j} {}^2T_{a,i,c,k} V_{j,b,k,c} \quad (407)$$

$$\tau^0_{\alpha,i} = \sum_{a \in V} {}^1T_{a,i} W^2_{a,\alpha} \quad (2r_V N_o N_v) \quad (408)$$

$$\tau^1_{\alpha} = \sum_{i \in O} W^1_{i,\alpha} \tau^0_{\alpha,i} \quad (2r_V N_o) \quad (409)$$

$$\tau^2_{\alpha} = \sum_{\beta \in B} \tau^1_{\beta} X_{\beta,\alpha} \quad (2r_V^2) \quad (410)$$

$$\tau^3_{i,a} = \sum_{\alpha \in B} \tau^2_{\alpha} W^3_{i,\alpha} W^4_{a,\alpha} \quad (3r_V N_o N_v) \quad (411)$$

$$\tau^4_{\gamma,i} = \sum_{a \in V} Y^3_{a,\gamma} \tau^3_{i,a} \quad (2r_T N_o N_v) \quad (412)$$

$$\tau^5_{\gamma} = \sum_{i \in O} Y^4_{i,\gamma} \tau^4_{\gamma,i} \quad (2r_T N_o) \quad (413)$$

$$\tau^6_{\gamma} = \sum_{\delta \in A} \tau^5_p Z_{\gamma,\delta} \quad (2r_T^2) \quad (414)$$

$${}^1R_{a,i} \leftarrow \sum_{\gamma \in A} 2 \tau^6_{\gamma} Y^1_{a,\gamma} Y^2_{i,\gamma} \quad (3r_T N_o N_v) \quad (415)$$

Raw expression

$${}^1R_{a,i} \leftarrow \sum_{j \in O} \sum_{k \in O} \sum_{b \in V} \sum_{c \in V} 2 {}^1T_{b,j} {}^2T_{c,k,a,i} V_{j,b,k,c} \quad (416)$$

Factorized expression

$$\tau^0_{\alpha,i} = \sum_{a \in V} {}^1T_{a,i} W^2_{a,\alpha} \quad (2r_V N_o N_v) \quad (417)$$

$$\tau^1_{\alpha} = \sum_{i \in O} W^1_{i,\alpha} \tau^0_{\alpha,i} \quad (2r_V N_o) \quad (418)$$

$$\tau^2_{\alpha} = \sum_{\beta \in B} \tau^1_{\beta} X_{\beta,\alpha} \quad (2r_V^2) \quad (419)$$

$$\tau^3_{i,a} = \sum_{\alpha \in B} \tau^2_{\alpha} W^3_{i,\alpha} W^4_{a,\alpha} \quad (3r_V N_o N_v) \quad (420)$$

$$\tau^4_{\gamma,i} = \sum_{a \in V} Y^1_{a,\gamma} \tau^3_{i,a} \quad (2r_T N_o N_v) \quad (421)$$

$$\tau^5_{\gamma} = \sum_{i \in O} Y^2_{i,\gamma} \tau^4_{\gamma,i} \quad (2r_T N_o) \quad (422)$$

$$\tau^6_{\gamma} = \sum_{\delta \in A} \tau^5_p Z_{\delta,\gamma} \quad (2r_T^2) \quad (423)$$

$${}^1R_{a,i} \leftarrow \sum_{\gamma \in A} 2 \tau^6_{\gamma} Y^3_{a,\gamma} Y^4_{i,\gamma} \quad (3r_T N_o N_v) \quad (424)$$

## VII. THC-RCCSD DOUBLES ( $Y^1$ FACTOR) EQUATION

Here expressions for a THC-RCCSD doubles residual, projected against all factors except  $Y^1$ , are given along with their cost

### A. Contributions from $H$

Raw expression

$${}^{21}R_{a,\epsilon} \leftarrow \sum_{\gamma \in A} \sum_{i \in O} \sum_{j \in O} \sum_{b \in V} Y^{2,*}_{i,\epsilon} Z^*_{\epsilon,\gamma} Y^{3,*}_{b,\gamma} Y^{4,*}_{j,\gamma} {}^2D^{a,i,b,j}_{V_{a,i,b,j}} \quad (425)$$

Factorized expression

$$\tau^0_{\gamma,\alpha,w} = \sum_{i \in O} {}^2D^2_{i,w} W^2_{i,\alpha} Y^{2,*}_{i,\gamma} \quad (3r_D r_T r_V N_o) \quad (426)$$

$$\tau^1_{\gamma,\alpha,w} = \sum_{a \in V} {}^2D^3_{a,w} W^3_{a,\alpha} Y^{3,*}_{a,\gamma} \quad (3r_D r_T r_V N_v) \quad (427)$$

$$\tau^2_{\gamma,\alpha,w} = \sum_{i \in O} {}^2D^4_{i,w} W^4_{i,\alpha} Y^{4,*}_{i,\gamma} \quad (3r_D r_T r_V N_o) \quad (428)$$

$$\tau^3_{\gamma,\alpha,w} = \sum_{\beta \in B} X_{\alpha,\beta} \tau^1_{\gamma,\beta,w} \tau^2_{\gamma,\beta,w} \quad (3r_D r_T r_V^2) \quad (429)$$

$$\tau^4_{\gamma,\alpha,w} = \sum_{\delta \in A} Z^*_{\gamma,\delta} \tau^3_{\delta,\alpha,w} \quad (2r_D r_T^2 r_V) \quad (430)$$

$$\tau^5_{\gamma,w,a} = \sum_{\alpha \in B} W^1_{a,\alpha} \tau^0_{\gamma,\alpha,w} \tau^4_{\gamma,\alpha,w} \quad (3r_D r_T r_V N_v) \quad (431)$$

$${}^{21}R_{a,\gamma} \leftarrow \sum_{w \in D} {}^2D^1_{a,w} \tau^5_{\gamma,w,a} \quad (2r_D r_T N_v) \quad (432)$$

### B. Contributions from $(H^1 T)_c$

Raw expression

$${}^{21}R_{a,\epsilon} \leftarrow - \sum_{\gamma \in A} \sum_{i \in O} \sum_{j \in O} \sum_{k \in O} \sum_{b \in V} {}^1T_{a,k} Y^{2,*}_{i,\epsilon} Z^*_{\epsilon,\gamma} Y^{3,*}_{b,\gamma} Y^{4,*}_{j,\gamma} {}^2D^{a,i,b,j}_{V_{b,j,k,i}} \quad (433)$$

Factorized expression

$$\tau^0_{\alpha,i} = \sum_{a \in V} {}^1T_{a,i} W^2_{a,\alpha} \quad (2r_V N_o N_v) \quad (434)$$

$$\tau^1_{\gamma,\alpha,w} = \sum_{i \in O} {}^2D^2_{i,w} Y^{2,*}_{i,\gamma} \tau^0_{\alpha,i} \quad (3r_D r_T r_V N_o) \quad (435)$$

$$\tau^2_{\gamma,\alpha,w} = \sum_{a \in V} {}^2D^3_{a,w} W^3_{a,\alpha} Y^{3,*}_{a,\gamma} \quad (3r_D r_T r_V N_v) \quad (436)$$

$$\tau^3_{\gamma,\alpha,w} = \sum_{i \in O} {}^2D^4_{i,w} W^4_{i,\alpha} Y^{4,*}_{i,\gamma} \quad (3r_D r_T r_V N_o) \quad (437)$$

$$\tau^4_{\gamma,\alpha,w} = \sum_{\beta \in B} X_{\alpha,\beta} \tau^2_{\gamma,\beta,w} \tau^3_{\gamma,\beta,w} \quad (3r_D r_T r_V^2) \quad (438)$$

$$\tau^5_{\gamma,\alpha,w} = \sum_{\delta \in A} Z^*_{\gamma,\delta} \tau^4_{\delta,\alpha,w} \quad (2r_D r_T^2 r_V) \quad (439)$$

$$\tau^6_{\gamma,w,a} = \sum_{\alpha \in B} W^1_{a,\alpha} \tau^1_{\gamma,\alpha,w} \tau^5_{\gamma,\alpha,w} \quad (3r_D r_T r_V N_v) \quad (440)$$

$${}^{21}R_{a,\gamma} \leftarrow \sum_{w \in D} {}^2D^1_{a,w} \tau^6_{\gamma,w,a} \quad (2r_D r_T N_v) \quad (441)$$

Raw expression

$${}^{21}R_{a,\epsilon} \leftarrow - \sum_{\gamma \in A} \sum_{i \in O} \sum_{j \in O} \sum_{k \in O} \sum_{b \in V} {}^1T_{b,k} Y^{2,*}_{i,\epsilon} Z^*_{\epsilon,\gamma} Y^{3,*}_{b,\gamma} Y^{4,*}_{j,\gamma} {}^2D^{a,i,b,j}_{V_{a,i,k,j}} \quad (442)$$

Factorized expression

$$\tau^0_{\gamma,\alpha,w} = \sum_{i \in O} {}^2D^2_{i,w} W^2_{i,\alpha} Y^{2,*}_{i,\gamma} \quad (3r_D r_T r_V N_o) \quad (443)$$

$$\tau^1_{\alpha,i} = \sum_{a \in V} {}^1T_{a,i} W^4_{a,\alpha} \quad (2r_V N_o N_v) \quad (444)$$

$$\tau^2_{\gamma,\alpha,w} = \sum_{i \in O} {}^2D^4_{i,w} Y^{4,*}_{i,\gamma} \tau^1_{\alpha,i} \quad (3r_D r_T r_V N_o) \quad (445)$$

$$\tau^3_{\gamma,\alpha,w} = \sum_{a \in V} {}^2D^3_{a,w} W^3_{a,\alpha} Y^{3,*}_{a,\gamma} \quad (3r_D r_T r_V N_v) \quad (446)$$

$$\tau^4_{\gamma,\alpha,w} = \sum_{\beta \in B} X_{\alpha,\beta} \tau^2_{\gamma,\beta,w} \tau^3_{\gamma,\beta,w} \quad (3r_D r_T r_V^2) \quad (447)$$

$$\tau^5_{\gamma,\alpha,w} = \sum_{\delta \in A} Z^*_{\gamma,\delta} \tau^4_{\delta,\alpha,w} \quad (2r_D r_T^2 r_V) \quad (448)$$

$$\tau^6_{\gamma,w,a} = \sum_{\alpha \in B} W^1_{a,\alpha} \tau^0_{\gamma,\alpha,w} \tau^5_{\gamma,\alpha,w} \quad (3r_D r_T r_V N_v) \quad (449)$$

$${}^{21}R_{a,\gamma} \leftarrow \sum_{w \in D} {}^2D^1_{a,w} \tau^6_{\gamma,w,a} \quad (2r_D r_T N_v) \quad (450)$$

Raw expression

$${}^{21}R_{a,\epsilon} \leftarrow \sum_{\gamma \in A} \sum_{i \in O} \sum_{j \in O} \sum_{b \in V} \sum_{c \in V} {}^1T_{c,i} Y^{2,*}_{i,\epsilon} Z^*_{\epsilon,\gamma} Y^{3,*}_{b,\gamma} Y^{4,*}_{j,\gamma} {}^2D^{a,i,b,j}_{a,c,b,j} V_{a,c,b,j} \quad (451)$$

Factorized expression

$$\tau^0_{\gamma,\alpha,w} = \sum_{a \in V} {}^2D^3_{a,w} W^1_{a,\alpha} Y^{3,*}_{a,\gamma} \quad (3r_D r_T r_V N_v) \quad (452)$$

$$\tau^1_{\gamma,\alpha,w} = \sum_{i \in O} {}^2D^4_{i,w} W^2_{i,\alpha} Y^{4,*}_{i,\gamma} \quad (3r_D r_T r_V N_o) \quad (453)$$

$$\tau^2_{\gamma,\alpha,w} = \sum_{\beta \in B} X_{\beta,\alpha} \tau^0_{\gamma,\beta,w} \tau^1_{\gamma,\beta,w} \quad (3r_D r_T r_V^2) \quad (454)$$

$$\tau^3_{\gamma,\alpha,w} = \sum_{\delta \in A} Z^*_{\gamma,\delta} \tau^2_{\delta,\alpha,w} \quad (2r_D r_T^2 r_V) \quad (455)$$

$$\tau^4_{\gamma,\alpha,w} = \sum_{i \in O} {}^2D^2_{i,w} W^4_{i,\alpha} Y^{2,*}_{i,\gamma} \quad (3r_D r_T r_V N_o) \quad (456)$$

$$\tau^5_{\gamma,w,i} = \sum_{\alpha \in B} W^3_{i,\alpha} \tau^3_{\gamma,\alpha,w} \tau^4_{\gamma,\alpha,w} \quad (3r_D r_T r_V N_o) \quad (457)$$

$${}^{21}R_{a,\gamma} \leftarrow - \sum_{w \in D} \sum_{i \in O} {}^2D^1_{a,w} {}^1T_{a,i} \tau^5_{\gamma,w,i} \quad (3r_D r_T N_o N_v) \quad (458)$$

Raw expression

$${}^{21}R_{a,\epsilon} \leftarrow \sum_{\gamma \in A} \sum_{i \in O} \sum_{j \in O} \sum_{b \in V} \sum_{c \in V} {}^1T_{c,j} Y^{2,*}_{i,\epsilon} Z^*_{\epsilon,\gamma} Y^{3,*}_{b,\gamma} Y^{4,*}_{j,\gamma} {}^2D^{a,i,b,j}_{a,i,b,c} V_{a,i,b,c} \quad (459)$$

Factorized expression

$$\tau^0_{\gamma,\alpha,w} = \sum_{i \in O} {}^2D^2_{i,w} W^2_{i,\alpha} Y^{2,*}_{i,\gamma} \quad (3r_D r_T r_V N_o) \quad (460)$$

$$\tau^1_{\gamma,w,i} = \sum_{a \in V} {}^2D^3_{a,w} {}^1T_{a,i} Y^{3,*}_{a,\gamma} \quad (3r_D r_T N_o N_v) \quad (461)$$

$$\tau^2_{\gamma,\alpha,w} = \sum_{i \in O} W^3_{i,\alpha} \tau^1_{\gamma,w,i} \quad (2r_D r_T r_V N_o) \quad (462)$$

$$\tau^3_{\gamma,\alpha,w} = \sum_{i \in O} {}^2D^4_{i,w} W^4_{i,\alpha} Y^{4,*}_{i,\gamma} \quad (3r_D r_T r_V N_o) \quad (463)$$

$$\tau^4_{\gamma,\alpha,w} = \sum_{\beta \in B} X_{\alpha,\beta} \tau^2_{\gamma,\beta,w} \tau^3_{\gamma,\beta,w} \quad (3r_D r_T r_V^2) \quad (464)$$

$$\tau^5_{\gamma,\alpha,w} = \sum_{\delta \in A} Z^*_{\gamma,\delta} \tau^4_{\delta,\alpha,w} \quad (2r_D r_T^2 r_V) \quad (465)$$

$$\tau^6_{\gamma,w,a} = \sum_{\alpha \in B} W^1_{a,\alpha} \tau^0_{\gamma,\alpha,w} \tau^5_{\gamma,\alpha,w} \quad (3r_D r_T r_V N_v) \quad (466)$$

$${}^{21}R_{a,\gamma} \leftarrow - \sum_{w \in D} {}^2D^1_{a,w} \tau^6_{\gamma,w,a} \quad (2r_D r_T N_v) \quad (467)$$

### C. Contributions from $(H^1 T^1 T)_c$

Raw expression

$${}^{21}R_{a,\epsilon} \leftarrow - \sum_{\gamma \in A} \sum_{i \in O} \sum_{j \in O} \sum_{k \in O} \sum_{b \in V} \sum_{c \in V} {}^1T_{a,k} {}^1T_{c,i} Y^{2,*}_{i,\epsilon} Z^*_{\epsilon,\gamma} Y^{3,*}_{b,\gamma} Y^{4,*}_{j,\gamma} {}^2D^{a,i,b,j}_{b,j,k,c} V_{b,j,k,c} \quad (468)$$

Factorized expression

$$\tau^0_{\alpha,i} = \sum_{a \in V} {}^1T_{a,i} W^2_{a,\alpha} \quad (2r_V N_o N_v) \quad (469)$$

$$\tau^1_{\gamma,\alpha,w} = \sum_{i \in O} {}^2D^2_{i,w} Y^{2,*}_{i,\gamma} \tau^0_{\alpha,i} \quad (3r_D r_T r_V N_o) \quad (470)$$

$$\tau^2_{\alpha,i} = \sum_{a \in V} {}^1T_{a,i} W^4_{a,\alpha} \quad (2r_V N_o N_v) \quad (471)$$

$$\tau^3_{\gamma,\alpha,w} = \sum_{i \in O} {}^2D^4_{i,w} Y^{4,*}_{i,\gamma} \tau^2_{\alpha,i} \quad (3r_D r_T r_V N_o) \quad (472)$$

$$\tau^4_{\gamma,\alpha,w} = \sum_{a \in V} {}^2D^3_{a,w} W^3_{a,\alpha} Y^{3,*}_{a,\gamma} \quad (3r_D r_T r_V N_v) \quad (473)$$

$$\tau^5_{\gamma,\alpha,w} = \sum_{\beta \in B} X_{\alpha,\beta} \tau^3_{\gamma,\beta,w} \tau^4_{\gamma,\beta,w} \quad (3r_D r_T r_V^2) \quad (474)$$

$$\tau^6_{\gamma,\alpha,w} = \sum_{\delta \in A} Z^*_{\gamma,\delta} \tau^5_{\delta,\alpha,w} \quad (2r_D r_T^2 r_V) \quad (475)$$

$$\tau^7_{\gamma,w,a} = \sum_{\alpha \in B} W^1_{a,\alpha} \tau^1_{\gamma,\alpha,w} \tau^6_{\gamma,\alpha,w} \quad (3r_D r_T r_V N_v) \quad (476)$$

$${}^{21}R_{a,\gamma} \leftarrow \sum_{w \in D} {}^2D^1_{a,w} \tau^7_{\gamma,w,a} \quad (2r_D r_T N_v) \quad (477)$$

Raw expression

$${}^{21}R_{a,\epsilon} \leftarrow - \sum_{\gamma \in A} \sum_{i \in O} \sum_{j \in O} \sum_{k \in O} \sum_{b \in V} \sum_{c \in V} {}^1T_{a,k} {}^1T_{c,j} Y^{2,*}_{i,\epsilon} Z^*_{\epsilon,\gamma} Y^{3,*}_{b,\gamma} Y^{4,*}_{j,\gamma} {}^2D^{a,i,b,j}_{b,c,k,i} \quad (478)$$

Factorized expression

$$\tau^0_{\gamma,\alpha,w} = \sum_{i \in O} {}^2D^2_{i,w} W^2_{i,\alpha} Y^{2,*}_{i,\gamma} \quad (3r_D r_T r_V N_o) \quad (479)$$

$$\tau^1_{\gamma,w,i} = \sum_{a \in V} {}^2D^3_{a,w} {}^1T_{a,i} Y^{3,*}_{a,\gamma} \quad (3r_D r_T N_o N_v) \quad (480)$$

$$\tau^2_{\gamma,\alpha,w} = \sum_{i \in O} W^3_{i,\alpha} \tau^1_{\gamma,w,i} \quad (2r_D r_T r_V N_o) \quad (481)$$

$$\tau^3_{\gamma,\alpha,w} = \sum_{i \in O} {}^2D^4_{i,w} W^4_{i,\alpha} Y^{4,*}_{i,\gamma} \quad (3r_D r_T r_V N_o) \quad (482)$$

$$\tau^4_{\gamma,\alpha,w} = \sum_{\beta \in B} X_{\alpha,\beta} \tau^2_{\gamma,\beta,w} \tau^3_{\gamma,\beta,w} \quad (3r_D r_T r_V^2) \quad (483)$$

$$\tau^5_{\gamma,\alpha,w} = \sum_{\delta \in A} Z^*_{\gamma,\delta} \tau^4_{\delta,\alpha,w} \quad (2r_D r_T^2 r_V) \quad (484)$$

$$\tau^6_{\gamma,w,i} = \sum_{\alpha \in B} W^1_{i,\alpha} \tau^0_{\gamma,\alpha,w} \tau^5_{\gamma,\alpha,w} \quad (3r_D r_T r_V N_o) \quad (485)$$

$${}^{21}R_{a,\gamma} \leftarrow \sum_{w \in D} \sum_{i \in O} {}^2D^1_{a,w} {}^1T_{a,i} \tau^6_{\gamma,w,i} \quad (3r_D r_T N_o N_v) \quad (486)$$

Raw expression

$${}^{21}R_{a,\epsilon} \leftarrow - \sum_{\gamma \in A} \sum_{i \in O} \sum_{j \in O} \sum_{k \in O} \sum_{b \in V} \sum_{c \in V} {}^1T_{b,k} {}^1T_{c,i} Y^{2,*}_{i,\epsilon} Z^*_{\epsilon,\gamma} Y^{3,*}_{b,\gamma} Y^{4,*}_{j,\gamma} {}^2D^{a,i,b,j}_{b,c,k,j} \quad (487)$$

Factorized expression

$$\tau^0_{\alpha,i} = \sum_{a \in V} {}^1T_{a,i} W^4_{a,\alpha} \quad (2r_V N_o N_v) \quad (488)$$

$$\tau^1_{\gamma,\alpha,w} = \sum_{i \in O} {}^2D^2_{i,w} Y^{2,*}_{i,\gamma} \tau^0_{\alpha,i} \quad (3r_D r_T r_V N_o) \quad (489)$$

$$\tau^2_{\gamma,\alpha,w} = \sum_{a \in V} {}^2D^3_{a,w} W^1_{a,\alpha} Y^{3,*}_{a,\gamma} \quad (3r_D r_T r_V N_v) \quad (490)$$

$$\tau^3_{\gamma,\alpha,w} = \sum_{i \in O} {}^2D^4_{i,w} W^2_{i,\alpha} Y^{4,*}_{i,\gamma} \quad (3r_D r_T r_V N_o) \quad (491)$$

$$\tau^4_{\gamma,\alpha,w} = \sum_{\beta \in B} X_{\beta,\alpha} \tau^2_{\gamma,\beta,w} \tau^3_{\gamma,\beta,w} \quad (3r_D r_T r_V^2) \quad (492)$$

$$\tau^5_{\gamma,\alpha,w} = \sum_{\delta \in A} Z^*_{\gamma,\delta} \tau^4_{\delta,\alpha,w} \quad (2r_D r_T^2 r_V) \quad (493)$$

$$\tau^6_{\gamma,w,i} = \sum_{\alpha \in B} W^3_{i,\alpha} \tau^1_{\gamma,\alpha,w} \tau^5_{\gamma,\alpha,w} \quad (3r_D r_T r_V N_o) \quad (494)$$

$$^{21}R_{a,\gamma} \leftarrow - \sum_{w \in D} \sum_{i \in O} {}^2D^1_{a,w} {}^1T_{a,i} \tau^6_{\gamma,w,i} \quad (3r_D r_T N_o N_v) \quad (495)$$

Raw expression

$$^{21}R_{a,\epsilon} \leftarrow - \sum_{\gamma \in A} \sum_{i \in O} \sum_{j \in O} \sum_{k \in O} \sum_{b \in V} \sum_{c \in V} {}^1T_{b,k} {}^1T_{c,j} Y^{2,*}_{i,\epsilon} Z^*_{\epsilon,\gamma} Y^{3,*}_{b,\gamma} Y^{4,*}_{j,\gamma} {}^2D^{a,i,b,j}_{a,i,k,c} V_{a,i,k,c} \quad (496)$$

Factorized expression

$$\tau^0_{\gamma,\alpha,w} = \sum_{i \in O} {}^2D^2_{i,w} W^4_{i,\alpha} Y^{2,*}_{i,\gamma} \quad (3r_D r_T r_V N_o) \quad (497)$$

$$\tau^1_{\alpha,i} = \sum_{a \in V} {}^1T_{a,i} W^2_{a,\alpha} \quad (2r_V N_o N_v) \quad (498)$$

$$\tau^2_{\gamma,\alpha,w} = \sum_{i \in O} {}^2D^4_{i,w} Y^{4,*}_{i,\gamma} \tau^1_{\alpha,i} \quad (3r_D r_T r_V N_o) \quad (499)$$

$$\tau^3_{\gamma,\alpha,w} = \sum_{a \in V} {}^2D^3_{a,w} W^1_{a,\alpha} Y^{3,*}_{a,\gamma} \quad (3r_D r_T r_V N_v) \quad (500)$$

$$\tau^4_{\gamma,\alpha,w} = \sum_{\beta \in B} X_{\beta,\alpha} \tau^2_{\gamma,\beta,w} \tau^3_{\gamma,\beta,w} \quad (3r_D r_T r_V^2) \quad (501)$$

$$\tau^5_{\gamma,\alpha,w} = \sum_{\delta \in A} Z^*_{\gamma,\delta} \tau^4_{\delta,\alpha,w} \quad (2r_D r_T^2 r_V) \quad (502)$$

$$\tau^6_{\gamma,w,i} = \sum_{\alpha \in B} W^3_{i,\alpha} \tau^0_{\gamma,\alpha,w} \tau^5_{\gamma,\alpha,w} \quad (3r_D r_T r_V N_o) \quad (503)$$

$$^{21}R_{a,\gamma} \leftarrow - \sum_{w \in D} \sum_{i \in O} {}^2D^1_{a,w} {}^1T_{a,i} \tau^6_{\gamma,w,i} \quad (3r_D r_T N_o N_v) \quad (504)$$

Raw expression

$$^{21}R_{a,\epsilon} \leftarrow \sum_{\gamma \in A} \sum_{i \in O} \sum_{j \in O} \sum_{k \in O} \sum_{l \in O} \sum_{b \in V} {}^1T_{a,k} {}^1T_{b,l} Y^{2,*}_{i,\epsilon} Z^*_{\epsilon,\gamma} Y^{3,*}_{b,\gamma} Y^{4,*}_{j,\gamma} {}^2D^{a,i,b,j}_{k,i,l,j} V_{k,i,l,j} \quad (505)$$

Factorized expression

$$\tau^0_{\alpha,i} = \sum_{a \in V} {}^1T_{a,i} W^2_{a,\alpha} \quad (2r_V N_o N_v) \quad (506)$$

$$\tau^1_{\gamma,\alpha,w} = \sum_{i \in O} {}^2D^2_{i,w} Y^{2,*}_{i,\gamma} \tau^0_{\alpha,i} \quad (3r_D r_T r_V N_o) \quad (507)$$

$$\tau^2_{\gamma,w,i} = \sum_{a \in V} {}^2D^3_{a,w} {}^1T_{a,i} Y^{3,*}_{a,\gamma} \quad (3r_D r_T N_o N_v) \quad (508)$$

$$\tau^3_{\gamma,\alpha,w} = \sum_{i \in O} W^3_{i,\alpha} \tau^2_{\gamma,w,i} \quad (2r_D r_T r_V N_o) \quad (509)$$

$$\tau^4_{\gamma,\alpha,w} = \sum_{i \in O} {}^2D^4_{i,w} W^4_{i,\alpha} Y^{4,*}_{i,\gamma} \quad (3r_D r_T r_V N_o) \quad (510)$$

$$\tau^5_{\gamma,\alpha,w} = \sum_{\beta \in B} X_{\alpha,\beta} \tau^3_{\gamma,\beta,w} \tau^4_{\gamma,\beta,w} \quad (3r_D r_T r_V^2) \quad (511)$$

$$\tau^6_{\gamma,\alpha,w} = \sum_{\delta \in A} Z^*_{\gamma,\delta} \tau^5_{\delta,\alpha,w} \quad (2r_D r_T^2 r_V) \quad (512)$$

$$\tau^7_{\gamma,w,a} = \sum_{\alpha \in B} W^1_{a,\alpha} \tau^1_{\gamma,\alpha,w} \tau^6_{\gamma,\alpha,w} \quad (3r_D r_T r_V N_v) \quad (513)$$

$$^{21}R_{a,\gamma} \leftarrow - \sum_{w \in D} {}^2D^1_{a,w} \tau^7_{\gamma,w,a} \quad (2r_D r_T N_v) \quad (514)$$

Raw expression

$$^{21}R_{a,\epsilon} \leftarrow \sum_{\gamma \in A} \sum_{i \in O} \sum_{j \in O} \sum_{b \in V} \sum_{c \in V} \sum_{d \in V} {}^1T_{c,i} {}^1T_{d,j} Y^{2,*}_{i,\epsilon} Z^*_{\epsilon,\gamma} Y^{3,*}_{b,\gamma} Y^{4,*}_{j,\gamma} {}^2D^{a,i,b,j}_{c,a,b,d} V_{a,c,b,d} \quad (515)$$

Factorized expression

$$\tau^0_{\gamma,\alpha,w} = \sum_{i \in O} {}^2D^2_{i,w} W^2_{i,\alpha} Y^{2,*}_{i,\gamma} \quad (3r_D r_T r_V N_o) \quad (516)$$

$$\tau^1_{\alpha,i} = \sum_{a \in V} {}^1T_{a,i} W^4_{a,\alpha} \quad (2r_V N_o N_v) \quad (517)$$

$$\tau^2_{\gamma,\alpha,w} = \sum_{i \in O} {}^2D^4_{i,w} Y^{4,*}_{i,\gamma} \tau^1_{\alpha,i} \quad (3r_D r_T r_V N_o) \quad (518)$$

$$\tau^3_{\gamma,w,i} = \sum_{a \in V} {}^2D^3_{a,w} {}^1T_{a,i} Y^{3,*}_{a,\gamma} \quad (3r_D r_T N_o N_v) \quad (519)$$

$$\tau^4_{\gamma,\alpha,w} = \sum_{i \in O} W^3_{i,\alpha} \tau^3_{\gamma,w,i} \quad (2r_D r_T r_V N_o) \quad (520)$$

$$\tau^5_{\gamma,\alpha,w} = \sum_{\beta \in B} X_{\alpha,\beta} \tau^2_{\gamma,\beta,w} \tau^4_{\gamma,\beta,w} \quad (3r_D r_T r_V^2) \quad (521)$$

$$\tau^6_{\gamma,\alpha,w} = \sum_{\delta \in A} Z^*_{\gamma,\delta} \tau^5_{\delta,\alpha,w} \quad (2r_D r_T^2 r_V) \quad (522)$$

$$\tau^7_{\gamma,w,a} = \sum_{\alpha \in B} W^1_{a,\alpha} \tau^0_{\gamma,\alpha,w} \tau^6_{\gamma,\alpha,w} \quad (3r_D r_T r_V N_v) \quad (523)$$

$${}^{21}R_{a,\gamma} \leftarrow - \sum_{w \in D} {}^2D^1_{a,w} \tau^7_{\gamma,w,a} \quad (2r_D r_T N_v) \quad (524)$$

#### D. Contributions from $(H^2T)_c$

Raw expression

$${}^{21}R_{a,\epsilon} \leftarrow - \sum_{\gamma \in A} \sum_{i \in O} \sum_{j \in O} \sum_{k \in O} \sum_{b \in V} \frac{1}{2} Y^{2,*}_{i,\epsilon} Z^*_{\epsilon,\gamma} Y^{3,*}_{b,\gamma} Y^{4,*}_{j,\gamma} f_{k,i} {}^2D^{a,i,b,j} {}^2T_{a,k,b,j} \quad (525)$$

Factorized expression

$$\tau^0_{\gamma,\delta,w} = \sum_{i \in O} {}^2D^2_{i,w} Y^2_{i,\gamma} Y^{2,*}_{i,\delta} \quad (3r_D r_T^2 N_o) \quad (526)$$

$$\tau^1_{\gamma,\delta,w} = \sum_{i \in O} {}^2D^4_{i,w} Y^4_{i,\gamma} Y^{4,*}_{i,\delta} \quad (3r_D r_T^2 N_o) \quad (527)$$

$$\tau^2_{\gamma,a} = \sum_{b \in V} Y^3_{b,\gamma} f_{a,b} \quad (2r_T N_v^2) \quad (528)$$

$$\tau^3_{\gamma,\delta,w} = \sum_{a \in V} {}^2D^3_{a,w} Y^{3,*}_{a,\delta} \tau^2_{\gamma,a} \quad (3r_D r_T^2 N_v) \quad (529)$$

$$\tau^4_{\gamma,\delta,w} = \sum_{\epsilon \in A} Z^*_{\delta,\epsilon} \tau^1_{\gamma,\epsilon,w} \tau^3_{\gamma,\epsilon,w} \quad (3r_D r_T^3) \quad (530)$$

$$\tau^5_{\gamma,\delta,w} = \sum_{\epsilon \in A} Z_{\gamma,\epsilon} \tau^4_{\epsilon,\delta,w} \quad (2r_D r_T^3) \quad (531)$$

$${}^{21}R_{a,\gamma} \leftarrow \sum_{\delta \in A} \sum_{w \in D} \frac{1}{2} {}^2D^1_{a,w} Y^1_{a,\delta} \tau^0_{\delta,\gamma,w} \tau^5_{\delta,\gamma,w} \quad (4r_D r_T^2 N_v) \quad (532)$$

Raw expression

$${}^{21}R_{a,\epsilon} \leftarrow - \sum_{\gamma \in A} \sum_{i \in O} \sum_{j \in O} \sum_{k \in O} \sum_{b \in V} \frac{1}{2} Y^{2,*}_{i,\epsilon} Z^*_{\epsilon,\gamma} Y^{3,*}_{b,\gamma} Y^{4,*}_{j,\gamma} f_{k,i} {}^2D^{a,i,b,j} {}^2T_{b,j,a,k} \quad (533)$$

Factorized expression

$$\tau^0_{\gamma,\delta,w} = \sum_{a \in V} {}^2D^3_{a,w} Y^1_{a,\gamma} Y^{3,*}_{a,\delta} \quad (3r_D r_T^2 N_v) \quad (534)$$

$$\tau^1_{\gamma,\delta,w} = \sum_{i \in O} {}^2D^4_{i,w} Y^2_{i,\gamma} Y^{4,*}_{i,\delta} \quad (3r_D r_T^2 N_o) \quad (535)$$

$$\tau^2_{\gamma,\delta,w} = \sum_{\epsilon \in A} Z^*_{\delta,\epsilon} \tau^0_{\gamma,\epsilon,w} \tau^1_{\gamma,\epsilon,w} \quad (3r_D r_T^3) \quad (536)$$

$$\tau^3_{\gamma,\delta,w} = \sum_{\epsilon \in A} Z_{\epsilon,\gamma} \tau^2_{\epsilon,\delta,w} \quad (2r_D r_T^3) \quad (537)$$

$$\tau^4_{\gamma,\delta,w} = \sum_{i \in O} {}^2D^2_{i,w} Y^4_{i,\gamma} Y^{2,*}_{i,\delta} \quad (3r_D r_T^2 N_o) \quad (538)$$

$$\tau^5_{\gamma,a} = \sum_{b \in V} Y^3_{b,\gamma} f_{a,b} \quad (2r_T N_v^2) \quad (539)$$

$${}^{21}R_{a,\gamma} \leftarrow \sum_{\delta \in A} \sum_{w \in D} \frac{1}{2} {}^2D^1_{a,w} \tau^5_{\delta,a} \tau^3_{\delta,\gamma,w} \tau^4_{\delta,\gamma,w} \quad (4r_D r_T^2 N_v) \quad (540)$$

Raw expression

$${}^{21}R_{a,\epsilon} \leftarrow - \sum_{\gamma \in A} \sum_{i \in O} \sum_{j \in O} \sum_{k \in O} \sum_{b \in V} \frac{1}{2} Y^{2,*}_{i,\epsilon} Z^*_{\epsilon,\gamma} Y^{3,*}_{b,\gamma} Y^{4,*}_{j,\gamma} f_{k,j} {}^2D^{a,i,b,j} {}^2T_{a,i,b,k} \quad (541)$$

Factorized expression

$$\tau^0_{\gamma,\delta,w} = \sum_{i \in O} {}^2D^2_{i,w} Y^2_{i,\gamma} Y^{2,*}_{i,\delta} \quad (3r_D r_T^2 N_o) \quad (542)$$

$$\tau^5_{\gamma,\delta,w} = \sum_{i \in O} {}^2D^2_{i,w} Y^4_{i,\gamma} Y^{2,*}_{i,\delta} \quad (3r_D r_T^2 N_o) \quad (555)$$

$$\tau^1_{\gamma,\delta,w} = \sum_{a \in V} {}^2D^3_{a,w} Y^3_{a,\gamma} Y^{3,*}_{a,\delta} \quad (3r_D r_T^2 N_v) \quad (543)$$

$${}^{21}R_{a,\gamma} \leftarrow \sum_{\delta \in A} \sum_{w \in D} \frac{1}{2} {}^2D^1_{a,w} Y^3_{a,\delta} \tau^4_{\delta,\gamma,w} \tau^5_{\delta,\gamma,w} \quad (4r_D r_T^2 N_v) \quad (556)$$

$$\tau^2_{\gamma,\delta,w} = \sum_{i \in O} {}^2D^4_{i,w} Y^4_{i,\gamma} Y^{4,*}_{i,\delta} \quad (3r_D r_T^2 N_o) \quad (544)$$

Raw expression

$${}^{21}R_{a,\epsilon} \leftarrow \sum_{\gamma \in A} \sum_{i \in O} \sum_{j \in O} \sum_{k \in O} \sum_{l \in O} \sum_{b \in V} \frac{1}{2} Y^{2,*}_{i,\epsilon} Z^*_{\epsilon,\gamma} Y^{3,*}_{b,\gamma} Y^{4,*}_{j,\gamma} {}^2D^{a,i,b,j} {}^2T_{a,k,b,l} V_{k,i,l,j} \quad (557)$$

$$\tau^3_{\gamma,\delta,w} = \sum_{\epsilon \in A} Z^*_{\delta,\epsilon} \tau^1_{\gamma,\epsilon,w} \tau^2_{\gamma,\epsilon,w} \quad (3r_D r_T^3) \quad (545)$$

Factorized expression

$$\tau^4_{\gamma,\delta,w} = \sum_{\epsilon \in A} Z_{\gamma,\epsilon} \tau^3_{\epsilon,\delta,w} \quad (2r_D r_T^3) \quad (546)$$

$$\tau^0_{\gamma,\alpha} = \sum_{a \in V} W^2_{a,\alpha} Y^1_{a,\gamma} \quad (2r_T r_V N_v) \quad (558)$$

$$\tau^5_{\gamma,a} = \sum_{b \in V} Y^1_{b,\gamma} f_{a,b} \quad (2r_T N_v^2) \quad (547)$$

$$\tau^1_{\gamma,\alpha,a} = \sum_{\beta \in B} W^1_{a,\beta} X_{\beta,\alpha} \tau^0_{\gamma,\beta} \quad (3r_T r_V^2 N_v) \quad (559)$$

$${}^{21}R_{a,\gamma} \leftarrow \sum_{\delta \in A} \sum_{w \in D} \frac{1}{2} {}^2D^1_{a,w} \tau^5_{\delta,a} \tau^0_{\delta,\gamma,w} \tau^4_{\delta,\gamma,w} \quad (4r_D r_T^2 N_v) \quad (548)$$

$$\tau^2_{\gamma,\alpha,w} = \sum_{a \in V} {}^2D^3_{a,w} W^3_{a,\alpha} Y^{3,*}_{a,\gamma} \quad (3r_D r_T r_V N_v) \quad (560)$$

Raw expression

$${}^{21}R_{a,\epsilon} \leftarrow - \sum_{\gamma \in A} \sum_{i \in O} \sum_{j \in O} \sum_{k \in O} \sum_{b \in V} \frac{1}{2} Y^{2,*}_{i,\epsilon} Z^*_{\epsilon,\gamma} Y^{3,*}_{b,\gamma} Y^{4,*}_{j,\gamma} f_{k,j} {}^2D^{a,i,b,j} {}^2T_{b,k,a,i} \quad (549)$$

$$\tau^3_{\gamma,\alpha} = \sum_{a \in V} W^4_{a,\alpha} Y^3_{a,\gamma} \quad (2r_T r_V N_v) \quad (561)$$

Factorized expression

$$\tau^4_{\gamma,\alpha,i} = \sum_{\delta \in A} Z_{\gamma,\delta} Y^4_{i,\delta} \tau^3_{\delta,\alpha} \quad (3r_T^2 r_V N_o) \quad (562)$$

$$\tau^0_{\gamma,\delta,w} = \sum_{i \in O} {}^2D^4_{i,w} Y^2_{i,\gamma} Y^{4,*}_{i,\delta} \quad (3r_D r_T^2 N_o) \quad (550)$$

$$\tau^5_{\gamma,\delta,\alpha,w} = \sum_{i \in O} {}^2D^4_{i,w} Y^{4,*}_{i,\delta} \tau^2_{\delta,\alpha,w} \tau^4_{\gamma,\alpha,i} \quad (4r_D r_T^2 r_V N_o) \quad (563)$$

$$\tau^1_{\gamma,a} = \sum_{b \in V} Y^1_{b,\gamma} f_{a,b} \quad (2r_T N_v^2) \quad (551)$$

$$\tau^6_{\gamma,\delta,w,a} = \sum_{\alpha \in B} \tau^1_{\gamma,\alpha,a} \tau^5_{\gamma,\delta,\alpha,w} \quad (2r_D r_T^2 r_V N_v) \quad (564)$$

$$\tau^2_{\gamma,\delta,w} = \sum_{a \in V} {}^2D^3_{a,w} Y^{3,*}_{a,\delta} \tau^1_{\gamma,a} \quad (3r_D r_T^2 N_v) \quad (552)$$

$$\tau^7_{\gamma,i,a} = \sum_{\delta \in A} \sum_{w \in D} {}^2D^1_{a,w} {}^2D^2_{i,w} Y^2_{i,\delta} \tau^6_{\delta,\gamma,w,a} \quad (4r_D r_T^2 N_o N_v) \quad (565)$$

$$\tau^3_{\gamma,\delta,w} = \sum_{\epsilon \in A} Z^*_{\delta,\epsilon} \tau^0_{\gamma,\epsilon,w} \tau^2_{\gamma,\epsilon,w} \quad (3r_D r_T^3) \quad (553)$$

$${}^{21}R_{a,\gamma} \leftarrow \sum_{\delta \in A} \sum_{i \in O} \frac{1}{2} Y^{2,*}_{i,\gamma} Z^*_{\gamma,\delta} \tau^7_{\delta,i,a} \quad (3r_T^2 N_o N_v) \quad (566)$$

$$\tau^4_{\gamma,\delta,w} = \sum_{\epsilon \in A} Z_{\epsilon,\gamma} \tau^3_{\epsilon,\delta,w} \quad (2r_D r_T^3) \quad (554)$$

Raw expression

$${}^{21}R_{a,\epsilon} \leftarrow \sum_{\gamma \in A} \sum_{i \in O} \sum_{j \in O} \sum_{k \in O} \sum_{l \in O} \sum_{b \in V} \frac{1}{2} Y^{2,*}_{i,\epsilon} Z^{*}_{\epsilon,\gamma} Y^{3,*}_{b,\gamma} Y^{4,*}_{j,\gamma} {}^2D^{a,i,b,j} {}^2T_{b,k,a,l} V_{l,i,k,j} \quad (567)$$

Factorized expression

$$\tau^0_{\gamma,\alpha} = \sum_{a \in V} W^2_{a,\alpha} Y^3_{a,\gamma} \quad (2r_T r_V N_v) \quad (568)$$

$$\tau^1_{\gamma,\alpha,a} = \sum_{\beta \in B} W^1_{a,\beta} X_{\beta,\alpha} \tau^0_{\gamma,\beta} \quad (3r_T r_V^2 N_v) \quad (569)$$

$$\tau^2_{\gamma,\alpha,w} = \sum_{a \in V} {}^2D^3_{a,w} W^3_{a,\alpha} Y^{3,*}_{a,\gamma} \quad (3r_D r_T r_V N_v) \quad (570)$$

$$\tau^3_{\gamma,\alpha} = \sum_{a \in V} W^4_{a,\alpha} Y^1_{a,\gamma} \quad (2r_T r_V N_v) \quad (571)$$

$$\tau^4_{\gamma,\alpha,i} = \sum_{\delta \in A} Y^2_{i,\delta} Z_{\delta,\gamma} \tau^3_{\delta,\alpha} \quad (3r_T^2 r_V N_o) \quad (572)$$

$$\tau^5_{\gamma,\delta,\alpha,w} = \sum_{i \in O} {}^2D^4_{i,w} Y^{4,*}_{i,\delta} \tau^2_{\delta,\alpha,w} \tau^4_{\gamma,\alpha,i} \quad (4r_D r_T^2 r_V N_o) \quad (573)$$

$$\tau^6_{\gamma,\delta,w,a} = \sum_{\alpha \in B} \tau^1_{\gamma,\alpha,a} \tau^5_{\gamma,\delta,\alpha,w} \quad (2r_D r_T^2 r_V N_v) \quad (574)$$

$$\tau^7_{\gamma,i,a} = \sum_{\delta \in A} \sum_{w \in D} {}^2D^1_{a,w} {}^2D^2_{i,w} Y^4_{i,\delta} \tau^6_{\delta,\gamma,w,a} \quad (4r_D r_T^2 N_o N_v) \quad (575)$$

$${}^{21}R_{a,\gamma} \leftarrow \sum_{\delta \in A} \sum_{i \in O} \frac{1}{2} Y^{2,*}_{i,\gamma} Z^{*}_{\gamma,\delta} \tau^7_{\delta,i,a} \quad (3r_T^2 N_o N_v) \quad (576)$$

Raw expression

$${}^{21}R_{a,\epsilon} \leftarrow \sum_{\gamma \in A} \sum_{i \in O} \sum_{j \in O} \sum_{k \in O} \sum_{b \in V} \sum_{c \in V} Y^{2,*}_{i,\epsilon} Z^{*}_{\epsilon,\gamma} Y^{3,*}_{b,\gamma} Y^{4,*}_{j,\gamma} {}^2D^{a,i,b,j} {}^2T_{a,i,c,k} V_{b,j,k,c} \quad (577)$$

Factorized expression

$$\tau^0_{\gamma,\alpha,w} = \sum_{i \in O} {}^2D^2_{i,w} W^2_{i,\alpha} Y^{2,*}_{i,\gamma} \quad (3r_D r_T r_V N_o) \quad (578)$$

$$\tau^1_{\gamma,\alpha} = \sum_{a \in V} W^4_{a,\alpha} Y^3_{a,\gamma} \quad (2r_T r_V N_v) \quad (579)$$

$$\tau^2_{\gamma,\alpha} = \sum_{i \in O} W^3_{i,\alpha} Y^4_{i,\gamma} \quad (2r_T r_V N_o) \quad (580)$$

$$\tau^3_{\gamma,\alpha} = \sum_{\beta \in B} X_{\alpha,\beta} \tau^1_{\gamma,\beta} \tau^2_{\gamma,\beta} \quad (3r_T r_V^2) \quad (581)$$

$$\tau^4_{\gamma,\alpha} = \sum_{\delta \in A} Z_{\gamma,\delta} \tau^3_{\delta,\alpha} \quad (2r_T^2 r_V) \quad (582)$$

$$\tau^5_{\gamma,\delta,w} = \sum_{a \in V} {}^2D^3_{a,w} Y^1_{a,\gamma} Y^{3,*}_{a,\delta} \quad (3r_D r_T^2 N_v) \quad (583)$$

$$\tau^6_{\gamma,\delta,w} = \sum_{i \in O} {}^2D^4_{i,w} Y^2_{i,\gamma} Y^{4,*}_{i,\delta} \quad (3r_D r_T^2 N_o) \quad (584)$$

$$\tau^7_{\gamma,\delta,w} = \sum_{\epsilon \in A} Z^{*}_{\delta,\epsilon} \tau^5_{\gamma,\epsilon,w} \tau^6_{\gamma,\epsilon,w} \quad (3r_D r_T^3) \quad (585)$$

$$\tau^8_{\gamma,\alpha,w} = \sum_{\delta \in A} \tau^4_{\delta,\alpha} \tau^7_{\delta,\gamma,w} \quad (2r_D r_T^2 r_V) \quad (586)$$

$$\tau^9_{\gamma,w,a} = \sum_{\alpha \in B} W^1_{a,\alpha} \tau^0_{\gamma,\alpha,w} \tau^8_{\gamma,\alpha,w} \quad (3r_D r_T r_V N_v) \quad (587)$$

$${}^{21}R_{a,\gamma} \leftarrow \sum_{w \in D} {}^2D^1_{a,w} \tau^9_{\gamma,w,a} \quad (2r_D r_T N_v) \quad (588)$$

Raw expression

$${}^{21}R_{a,\epsilon} \leftarrow \sum_{\gamma \in A} \sum_{i \in O} \sum_{j \in O} \sum_{k \in O} \sum_{b \in V} \sum_{c \in V} Y^{2,*}_{i,\epsilon} Z^{*}_{\epsilon,\gamma} Y^{3,*}_{b,\gamma} Y^{4,*}_{j,\gamma} {}^2D^{a,i,b,j} {}^2T_{b,j,c,k} V_{a,i,k,c} \quad (589)$$

Factorized expression

$$\tau^0_{\gamma,\alpha,w} = \sum_{i \in O} {}^2D^2_{i,w} W^2_{i,\alpha} Y^{2,*}_{i,\gamma} \quad (3r_D r_T r_V N_o) \quad (590)$$

$$\tau^1_{\gamma,\delta,w} = \sum_{a \in V} {}^2D^3_{a,w} Y^3_{a,\gamma} Y^{3,*}_{a,\delta} \quad (3r_D r_T^2 N_v) \quad (591)$$



$$\tau^2_{\gamma,\delta,w} = \sum_{i \in O} {}^2D^4_{i,w} Y^4_{i,\gamma} Y^{4,*}_{i,\delta} \quad (3r_D r_T^2 N_o) \quad (592)$$

$$\tau^3_{\gamma,\delta,w} = \sum_{\epsilon \in A} Z^*_{\delta,\epsilon} \tau^1_{\gamma,\epsilon,w} \tau^2_{\gamma,\epsilon,w} \quad (3r_D r_T^3) \quad (593)$$

$$\tau^4_{\gamma,\alpha} = \sum_{a \in V} W^4_{a,\alpha} Y^1_{a,\gamma} \quad (2r_T r_V N_v) \quad (594)$$

$$\tau^5_{\gamma,\alpha} = \sum_{i \in O} W^3_{i,\alpha} Y^2_{i,\gamma} \quad (2r_T r_V N_o) \quad (595)$$

$$\tau^6_{\gamma,\alpha} = \sum_{\beta \in B} X_{\alpha,\beta} \tau^4_{\gamma,\beta} \tau^5_{\gamma,\beta} \quad (3r_T r_V^2) \quad (596)$$

$$\tau^7_{\gamma,\alpha} = \sum_{\delta \in A} Z_{\delta,\gamma} \tau^6_{\delta,\alpha} \quad (2r_T^2 r_V) \quad (597)$$

$$\tau^8_{\gamma,\alpha,w} = \sum_{\delta \in A} \tau^7_{\delta,\alpha} \tau^3_{\delta,\gamma,w} \quad (2r_D r_T^2 r_V) \quad (598)$$

$$\tau^9_{\gamma,w,a} = \sum_{\alpha \in B} W^1_{a,\alpha} \tau^0_{\gamma,\alpha,w} \tau^8_{\gamma,\alpha,w} \quad (3r_D r_T r_V N_v) \quad (599)$$

$${}^{21}R_{a,\gamma} \leftarrow \sum_{w \in D} {}^2D^1_{a,w} \tau^9_{\gamma,w,a} \quad (2r_D r_T N_v) \quad (600)$$

Raw expression

$${}^{21}R_{a,\epsilon} \leftarrow \sum_{\gamma \in A} \sum_{i \in O} \sum_{j \in O} \sum_{k \in O} \sum_{b \in V} \sum_{c \in V} Y^{2,*}_{i,\epsilon} Z^*_{\epsilon,\gamma} Y^{3,*}_{b,\gamma} Y^{4,*}_{j,\gamma} {}^2D^{a,i,b,j} {}^2T_{c,k,a,i} V_{b,j,k,c} \quad (601)$$

Factorized expression

$$\tau^0_{\gamma,\delta,w} = \sum_{i \in O} {}^2D^2_{i,w} Y^2_{i,\gamma} Y^{2,*}_{i,\delta} \quad (3r_D r_T^2 N_o) \quad (602)$$

$$\tau^1_{\gamma,\alpha,w} = \sum_{a \in V} {}^2D^3_{a,w} W^1_{a,\alpha} Y^{3,*}_{a,\gamma} \quad (3r_D r_T r_V N_v) \quad (603)$$

$$\tau^2_{\gamma,\alpha,w} = \sum_{i \in O} {}^2D^4_{i,w} W^2_{i,\alpha} Y^{4,*}_{i,\gamma} \quad (3r_D r_T r_V N_o) \quad (604)$$

$$\tau^3_{\gamma,\alpha} = \sum_{a \in V} W^4_{a,\alpha} Y^3_{a,\gamma} \quad (2r_T r_V N_v) \quad (605)$$

$$\tau^4_{\gamma,\alpha} = \sum_{i \in O} W^3_{i,\alpha} Y^4_{i,\gamma} \quad (2r_T r_V N_o) \quad (606)$$

$$\tau^5_{\gamma,\alpha} = \sum_{\beta \in B} X_{\alpha,\beta} \tau^3_{\gamma,\beta} \tau^4_{\gamma,\beta} \quad (3r_T r_V^2) \quad (607)$$

$$\tau^6_{\gamma,\alpha} = \sum_{\delta \in A} Z_{\gamma,\delta} \tau^5_{\delta,\alpha} \quad (2r_T^2 r_V) \quad (608)$$

$$\tau^7_{\gamma,\delta,w} = \sum_{\alpha \in B} \tau^6_{\gamma,\alpha} \tau^1_{\delta,\alpha,w} \tau^2_{\delta,\alpha,w} \quad (3r_D r_T^2 r_V) \quad (609)$$

$$\tau^8_{\gamma,\delta,w} = \sum_{\epsilon \in A} Z^*_{\delta,\epsilon} \tau^7_{\gamma,\epsilon,w} \quad (2r_D r_T^3) \quad (610)$$

$${}^{21}R_{a,\gamma} \leftarrow \sum_{\delta \in A} \sum_{w \in D} {}^2D^1_{a,w} Y^1_{a,\delta} \tau^0_{\delta,\gamma,w} \tau^8_{\delta,\gamma,w} \quad (4r_D r_T^2 N_v) \quad (611)$$

Raw expression

$${}^{21}R_{a,\epsilon} \leftarrow \sum_{\gamma \in A} \sum_{i \in O} \sum_{j \in O} \sum_{k \in O} \sum_{b \in V} \sum_{c \in V} Y^{2,*}_{i,\epsilon} Z^*_{\epsilon,\gamma} Y^{3,*}_{b,\gamma} Y^{4,*}_{j,\gamma} {}^2D^{a,i,b,j} {}^2T_{c,k,b,j} V_{a,i,k,c} \quad (612)$$

Factorized expression

$$\tau^0_{\gamma,\delta,w} = \sum_{i \in O} {}^2D^2_{i,w} Y^4_{i,\gamma} Y^{2,*}_{i,\delta} \quad (3r_D r_T^2 N_o) \quad (613)$$

$$\tau^1_{\gamma,\alpha,w} = \sum_{a \in V} {}^2D^3_{a,w} W^1_{a,\alpha} Y^{3,*}_{a,\gamma} \quad (3r_D r_T r_V N_v) \quad (614)$$

$$\tau^2_{\gamma,\alpha,w} = \sum_{i \in O} {}^2D^4_{i,w} W^2_{i,\alpha} Y^{4,*}_{i,\gamma} \quad (3r_D r_T r_V N_o) \quad (615)$$

$$\tau^3_{\gamma,\alpha} = \sum_{a \in V} W^4_{a,\alpha} Y^1_{a,\gamma} \quad (2r_T r_V N_v) \quad (616)$$

$$\tau^4_{\gamma,\alpha} = \sum_{i \in O} W^3_{i,\alpha} Y^2_{i,\gamma} \quad (2r_T r_V N_o) \quad (617)$$

$$\tau^5_{\gamma,\alpha} = \sum_{\beta \in B} X_{\alpha,\beta} \tau^3_{\gamma,\beta} \tau^4_{\gamma,\beta} \quad (3r_T r_V^2) \quad (618)$$

$$\tau^6_{\gamma,\alpha} = \sum_{\delta \in A} Z_{\delta,\gamma} \tau^5_{\delta,\alpha} \quad (2r_T^2 r_V) \quad (619)$$

$$\tau^7_{\gamma,\delta,w} = \sum_{\alpha \in B} \tau^6_{\gamma,\alpha} \tau^1_{\delta,\alpha,w} \tau^2_{\delta,\alpha,w} \quad (3r_D r_T^2 r_V) \quad (620)$$

$$\tau^8_{\gamma,\delta,w} = \sum_{\epsilon \in A} Z^*_{\delta,\epsilon} \tau^7_{\gamma,\epsilon,w} \quad (2r_D r_T^3) \quad (621)$$

$${}^{21}R_{a,\gamma} \leftarrow \sum_{\delta \in A} \sum_{w \in D} {}^2D^1_{a,w} Y^3_{a,\delta} \tau^0_{\delta,\gamma,w} \tau^8_{\delta,\gamma,w} \quad (4r_D r_T^2 N_v) \quad (622)$$

Raw expression

$${}^{21}R_{a,\epsilon} \leftarrow - \sum_{\gamma \in A} \sum_{i \in O} \sum_{j \in O} \sum_{k \in O} \sum_{b \in V} \sum_{c \in V} \frac{1}{2} Y^{2,*}_{i,\epsilon} Z^*_{\epsilon,\gamma} Y^{3,*}_{b,\gamma} Y^{4,*}_{j,\gamma} {}^2D^{a,i,b,j} {}^2T_{a,i,c,k} V_{b,c,k,j} \quad (623)$$

Factorized expression

$$\tau^0_{\gamma,\delta,w} = \sum_{a \in V} {}^2D^3_{a,w} Y^1_{a,\gamma} Y^{3,*}_{a,\delta} \quad (3r_D r_T^2 N_v) \quad (624)$$

$$\tau^1_{\gamma,\delta,w} = \sum_{i \in O} {}^2D^4_{i,w} Y^2_{i,\gamma} Y^{4,*}_{i,\delta} \quad (3r_D r_T^2 N_o) \quad (625)$$

$$\tau^2_{\gamma,\delta,w} = \sum_{\epsilon \in A} Z^*_{\delta,\epsilon} \tau^0_{\gamma,\epsilon,w} \tau^1_{\gamma,\epsilon,w} \quad (3r_D r_T^3) \quad (626)$$

$$\tau^3_{\gamma,\delta,w} = \sum_{\epsilon \in A} Z_{\epsilon,\gamma} \tau^2_{\epsilon,\delta,w} \quad (2r_D r_T^3) \quad (627)$$

$$\tau^4_{\alpha,i,j} = \sum_{\beta \in B} X_{\alpha,\beta} W^3_{i,\beta} W^4_{j,\beta} \quad (3r_V^2 N_o^2) \quad (628)$$

$$\tau^5_{\gamma,\alpha,i} = \sum_{j \in O} Y^4_{j,\gamma} \tau^4_{\alpha,j,i} \quad (2r_T r_V N_o^2) \quad (629)$$

$$\tau^6_{\gamma,\alpha} = \sum_{a \in V} W^2_{a,\alpha} Y^3_{a,\gamma} \quad (2r_T r_V N_v) \quad (630)$$

$$\tau^7_{\gamma,i,a} = \sum_{\alpha \in B} W^1_{a,\alpha} \tau^6_{\gamma,\alpha} \tau^5_{\gamma,\alpha,i} \quad (3r_T r_V N_o N_v) \quad (631)$$

$$\tau^8_{\gamma,w,a} = \sum_{\delta \in A} \sum_{i \in O} {}^2D^2_{i,w} Y^{2,*}_{i,\gamma} \tau^3_{\delta,\gamma,w} \tau^7_{\delta,i,a} \quad (4r_D r_T^2 N_o N_v) \quad (632)$$

$${}^{21}R_{a,\gamma} \leftarrow - \sum_{w \in D} \frac{1}{2} {}^2D^1_{a,w} \tau^8_{\gamma,w,a} \quad (2r_D r_T N_v) \quad (633)$$

Raw expression

$${}^{21}R_{a,\epsilon} \leftarrow - \sum_{\gamma \in A} \sum_{i \in O} \sum_{j \in O} \sum_{k \in O} \sum_{b \in V} \sum_{c \in V} \frac{1}{2} Y^{2,*}_{i,\epsilon} Z^*_{\epsilon,\gamma} Y^{3,*}_{b,\gamma} Y^{4,*}_{j,\gamma} {}^2D^{a,i,b,j} {}^2T_{a,k,c,i} V_{b,j,k,c} \quad (634)$$

Factorized expression

$$\tau^0_{\gamma,\delta,w} = \sum_{a \in V} {}^2D^3_{a,w} Y^3_{a,\gamma} Y^{3,*}_{a,\delta} \quad (3r_D r_T^2 N_v) \quad (635)$$

$$\tau^1_{\gamma,\delta,w} = \sum_{i \in O} {}^2D^4_{i,w} Y^4_{i,\gamma} Y^{4,*}_{i,\delta} \quad (3r_D r_T^2 N_o) \quad (636)$$

$$\tau^2_{\gamma,\delta,w} = \sum_{\epsilon \in A} Z^*_{\delta,\epsilon} \tau^0_{\gamma,\epsilon,w} \tau^1_{\gamma,\epsilon,w} \quad (3r_D r_T^3) \quad (637)$$

$$\tau^3_{\gamma,\delta,w} = \sum_{\epsilon \in A} Z_{\gamma,\epsilon} \tau^2_{\epsilon,\delta,w} \quad (2r_D r_T^3) \quad (638)$$

$$\tau^4_{\alpha,i,j} = \sum_{\beta \in B} X_{\alpha,\beta} W^3_{i,\beta} W^4_{j,\beta} \quad (3r_V^2 N_o^2) \quad (639)$$

$$\tau^5_{\gamma,\alpha,i} = \sum_{j \in O} Y^2_{j,\gamma} \tau^4_{\alpha,j,i} \quad (2r_T r_V N_o^2) \quad (640)$$

$$\tau^6_{\gamma,\alpha} = \sum_{a \in V} W^2_{a,\alpha} Y^1_{a,\gamma} \quad (2r_T r_V N_v) \quad (641)$$

$$\tau^7_{\gamma,i,a} = \sum_{\alpha \in B} W^1_{a,\alpha} \tau^6_{\gamma,\alpha} \tau^5_{\gamma,\alpha,i} \quad (3r_T r_V N_o N_v) \quad (642)$$

$$\tau^8_{\gamma,w,a} = \sum_{\delta \in A} \sum_{i \in O} {}^2D^2_{i,w} Y^{2,*}_{i,\gamma} \tau^3_{\delta,\gamma,w} \tau^7_{\delta,i,a} \quad (4r_D r_T^2 N_o N_v) \quad (643)$$

$${}^{21}R_{a,\gamma} \leftarrow - \sum_{w \in D} \frac{1}{2} {}^2D^1_{a,w} \tau^8_{\gamma,w,a} \quad (2r_D r_T N_v) \quad (644)$$

Raw expression

$${}^{21}R_{a,\epsilon} \leftarrow - \sum_{\gamma \in A} \sum_{i \in O} \sum_{j \in O} \sum_{k \in O} \sum_{b \in V} \sum_{c \in V} \frac{1}{2} Y^{2,*}_{i,\epsilon} Z^{*,\gamma}_{\epsilon,\gamma} Y^{3,*}_{b,\gamma} Y^{4,*}_{j,\gamma} {}^2D^{a,i,b,j} {}^2T_{a,k,c,j} V_{b,c,k,i} \quad (645)$$

Factorized expression

$$\tau^0_{\gamma,\alpha} = \sum_{a \in V} W^2_{a,\alpha} Y^3_{a,\gamma} \quad (2r_T r_V N_v) \quad (646)$$

$$\tau^1_{\gamma,\alpha,i} = \sum_{\delta \in A} Z_{\gamma,\delta} Y^4_{i,\delta} \tau^0_{\delta,\alpha} \quad (3r_T^2 r_V N_o) \quad (647)$$

$$\tau^2_{\gamma,\delta,w} = \sum_{a \in V} {}^2D^3_{a,w} Y^1_{a,\gamma} Y^{3,*}_{a,\delta} \quad (3r_D r_T^2 N_v) \quad (648)$$

$$\tau^3_{\gamma,\delta,w,i} = \sum_{\epsilon \in A} {}^2D^4_{i,w} Z^*_{\delta,\epsilon} Y^{4,*}_{i,\epsilon} \tau^2_{\gamma,\epsilon,w} \quad (4r_D r_T^3 N_o) \quad (649)$$

$$\tau^4_{\alpha,i,j} = \sum_{\beta \in B} X_{\alpha,\beta} W^3_{i,\beta} W^4_{j,\beta} \quad (3r_V^2 N_o^2) \quad (650)$$

$$\tau^5_{\gamma,\alpha,i} = \sum_{j \in O} Y^2_{j,\gamma} \tau^4_{\alpha,j,i} \quad (2r_T r_V N_o^2) \quad (651)$$

$$\tau^6_{\gamma,\delta,\alpha,w} = \sum_{i \in O} \tau^5_{\gamma,\alpha,i} \tau^3_{\gamma,\delta,w,i} \quad (2r_D r_T^2 r_V N_o) \quad (652)$$

$$\tau^7_{\gamma,\alpha,w,i} = \sum_{\delta \in A} \tau^1_{\delta,\alpha,i} \tau^6_{\delta,\gamma,\alpha,w} \quad (2r_D r_T^2 r_V N_o) \quad (653)$$

$$\tau^8_{\gamma,\alpha,w} = \sum_{i \in O} {}^2D^2_{i,w} Y^{2,*}_{i,\gamma} \tau^7_{\gamma,\alpha,w,i} \quad (3r_D r_T r_V N_o) \quad (654)$$

$$\tau^9_{\gamma,w,a} = \sum_{\alpha \in B} W^1_{a,\alpha} \tau^8_{\gamma,\alpha,w} \quad (2r_D r_T r_V N_v) \quad (655)$$

$${}^{21}R_{a,\gamma} \leftarrow - \sum_{w \in D} \frac{1}{2} {}^2D^1_{a,w} \tau^9_{\gamma,w,a} \quad (2r_D r_T N_v) \quad (656)$$

Raw expression

$${}^{21}R_{a,\epsilon} \leftarrow - \sum_{\gamma \in A} \sum_{i \in O} \sum_{j \in O} \sum_{k \in O} \sum_{b \in V} \sum_{c \in V} \frac{1}{2} Y^{2,*}_{i,\epsilon} Z^{*,\gamma}_{\epsilon,\gamma} Y^{3,*}_{b,\gamma} Y^{4,*}_{j,\gamma} {}^2D^{a,i,b,j} {}^2T_{b,j,c,k} V_{a,c,k,i} \quad (657)$$

Factorized expression

$$\tau^0_{\gamma,\delta,w} = \sum_{a \in V} {}^2D^3_{a,w} Y^3_{a,\gamma} Y^{3,*}_{a,\delta} \quad (3r_D r_T^2 N_v) \quad (658)$$

$$\tau^1_{\gamma,\delta,w,i} = \sum_{\epsilon \in A} {}^2D^4_{i,w} Z^*_{\delta,\epsilon} Y^{4,*}_{i,\epsilon} \tau^0_{\gamma,\epsilon,w} \quad (4r_D r_T^3 N_o) \quad (659)$$

$$\tau^2_{\alpha,i,j} = \sum_{\beta \in B} X_{\alpha,\beta} W^3_{i,\beta} W^4_{j,\beta} \quad (3r_V^2 N_o^2) \quad (660)$$

$$\tau^3_{\gamma,\alpha,i} = \sum_{j \in O} Y^4_{j,\gamma} \tau^2_{\alpha,j,i} \quad (2r_T r_V N_o^2) \quad (661)$$

$$\tau^4_{\gamma,\delta,\alpha,w} = \sum_{i \in O} \tau^3_{\gamma,\alpha,i} \tau^1_{\gamma,\delta,w,i} \quad (2r_D r_T^2 r_V N_o) \quad (662)$$

$$\tau^5_{\gamma,\alpha} = \sum_{a \in V} W^2_{a,\alpha} Y^1_{a,\gamma} \quad (2r_T r_V N_v) \quad (663)$$

$$\tau^6_{\gamma,\alpha,i} = \sum_{\delta \in A} Y^2_{i,\delta} Z_{\delta,\gamma} \tau^5_{\delta,\alpha} \quad (3r_T^2 r_V N_o) \quad (664)$$

$$\tau^7_{\gamma,\alpha,w,i} = \sum_{\delta \in A} \tau^6_{\delta,\alpha,i} \tau^4_{\delta,\gamma,\alpha,w} \quad (2r_D r_T^2 r_V N_o) \quad (665)$$

$$\tau^8_{\gamma,\alpha,w} = \sum_{i \in O} {}^2D^2_{i,w} Y^{2,*}_{i,\gamma} \tau^7_{\gamma,\alpha,w,i} \quad (3r_D r_T r_V N_o) \quad (666)$$

$$\tau^9_{\gamma,w,a} = \sum_{\alpha \in B} W^1_{a,\alpha} \tau^8_{\gamma,\alpha,w} \quad (2r_D r_T r_V N_v) \quad (667)$$

$${}^{21}R_{a,\gamma} \leftarrow - \sum_{w \in D} \frac{1}{2} {}^2D^1_{a,w} \tau^9_{\gamma,w,a} \quad (2r_D r_T N_v) \quad (668)$$

Raw expression

$${}^{21}R_{a,\epsilon} \leftarrow - \sum_{\gamma \in A} \sum_{i \in O} \sum_{j \in O} \sum_{k \in O} \sum_{b \in V} \sum_{c \in V} \frac{1}{2} Y^{2,*}_{i,\epsilon} Z^*_{\epsilon,\gamma} Y^{3,*}_{b,\gamma} Y^{4,*}_{j,\gamma} {}^2D^{a,i,b,j} {}^2T_{b,k,c,i} V_{a,c,k,j} \quad (669)$$

Factorized expression

$$\tau^0_{\gamma,\alpha,w} = \sum_{i \in O} {}^2D^2_{i,w} W^2_{i,\alpha} Y^{2,*}_{i,\gamma} \quad (3r_D r_T r_V N_o) \quad (670)$$

$$\tau^1_{\gamma,\delta,w} = \sum_{a \in V} {}^2D^3_{a,w} Y^1_{a,\gamma} Y^{3,*}_{a,\delta} \quad (3r_D r_T^2 N_v) \quad (671)$$

$$\tau^2_{\gamma,\alpha} = \sum_{i \in O} W^3_{i,\alpha} Y^2_{i,\gamma} \quad (2r_T r_V N_o) \quad (672)$$

$$\tau^3_{\gamma,\alpha} = \sum_{a \in V} W^4_{a,\alpha} Y^3_{a,\gamma} \quad (2r_T r_V N_v) \quad (673)$$

$$\tau^4_{\gamma,\alpha,i} = \sum_{\delta \in A} Z_{\gamma,\delta} Y^4_{i,\delta} \tau^3_{\delta,\alpha} \quad (3r_T^2 r_V N_o) \quad (674)$$

$$\tau^5_{\gamma,\alpha,w} = \sum_{\delta \in A} \sum_{i \in O} {}^2D^4_{i,w} Y^{4,*}_{i,\gamma} \tau^2_{\delta,\alpha} \tau^1_{\delta,\gamma,w} \tau^4_{\delta,\alpha,i} \quad (5r_D r_T^2 r_V N_o) \quad (675)$$

$$\tau^6_{\gamma,\alpha,w} = \sum_{\beta \in B} X_{\alpha,\beta} \tau^5_{\gamma,\beta,w} \quad (2r_D r_T r_V^2) \quad (676)$$

$$\tau^7_{\gamma,\alpha,w} = \sum_{\delta \in A} Z^*_{\gamma,\delta} \tau^6_{\delta,\alpha,w} \quad (2r_D r_T^2 r_V) \quad (677)$$

$$\tau^8_{\gamma,w,a} = \sum_{\alpha \in B} W^1_{a,\alpha} \tau^0_{\gamma,\alpha,w} \tau^7_{\gamma,\alpha,w} \quad (3r_D r_T r_V N_v) \quad (678)$$

$${}^{21}R_{a,\gamma} \leftarrow - \sum_{w \in D} \frac{1}{2} {}^2D^1_{a,w} \tau^8_{\gamma,w,a} \quad (2r_D r_T N_v) \quad (679)$$

Raw expression

$${}^{21}R_{a,\epsilon} \leftarrow - \sum_{\gamma \in A} \sum_{i \in O} \sum_{j \in O} \sum_{k \in O} \sum_{b \in V} \sum_{c \in V} \frac{1}{2} Y^{2,*}_{i,\epsilon} Z^*_{\epsilon,\gamma} Y^{3,*}_{b,\gamma} Y^{4,*}_{j,\gamma} {}^2D^{a,i,b,j} {}^2T_{b,k,c,j} V_{a,i,k,c} \quad (680)$$

Factorized expression

$$\tau^0_{\gamma,\alpha,w} = \sum_{i \in O} {}^2D^2_{i,w} W^2_{i,\alpha} Y^{2,*}_{i,\gamma} \quad (3r_D r_T r_V N_o) \quad (681)$$

$$\tau^1_{\gamma,\delta,w} = \sum_{a \in V} {}^2D^3_{a,w} Y^3_{a,\gamma} Y^{3,*}_{a,\delta} \quad (3r_D r_T^2 N_v) \quad (682)$$

$$\tau^2_{\gamma,\alpha} = \sum_{a \in V} W^4_{a,\alpha} Y^1_{a,\gamma} \quad (2r_T r_V N_v) \quad (683)$$

$$\tau^3_{\gamma,\alpha,i} = \sum_{\delta \in A} Y^2_{i,\delta} Z_{\delta,\gamma} \tau^2_{\delta,\alpha} \quad (3r_T^2 r_V N_o) \quad (684)$$

$$\tau^4_{\gamma,\alpha} = \sum_{i \in O} W^3_{i,\alpha} Y^4_{i,\gamma} \quad (2r_T r_V N_o) \quad (685)$$

$$\tau^5_{\gamma,\alpha,w} = \sum_{\delta \in A} \sum_{i \in O} {}^2D^4_{i,w} Y^{4,*}_{i,\gamma} \tau^4_{\delta,\alpha} \tau^1_{\delta,\gamma,w} \tau^3_{\delta,\alpha,i} \quad (5r_D r_T^2 r_V N_o) \quad (686)$$

$$\tau^6_{\gamma,\alpha,w} = \sum_{\beta \in B} X_{\alpha,\beta} \tau^5_{\gamma,\beta,w} \quad (2r_D r_T r_V^2) \quad (687)$$

$$\tau^7_{\gamma,\alpha,w} = \sum_{\delta \in A} Z^*_{\gamma,\delta} \tau^6_{\delta,\alpha,w} \quad (2r_D r_T^2 r_V) \quad (688)$$

$$\tau^8_{\gamma,w,a} = \sum_{\alpha \in B} W^1_{a,\alpha} \tau^0_{\gamma,\alpha,w} \tau^7_{\gamma,\alpha,w} \quad (3r_D r_T r_V N_v) \quad (689)$$

$${}^{21}R_{a,\gamma} \leftarrow - \sum_{w \in D} \frac{1}{2} {}^2D^1_{a,w} \tau^8_{\gamma,w,a} \quad (2r_D r_T N_v) \quad (690)$$

Raw expression

$${}^{21}R_{a,\epsilon} \leftarrow - \sum_{\gamma \in A} \sum_{i \in O} \sum_{j \in O} \sum_{k \in O} \sum_{b \in V} \sum_{c \in V} \frac{1}{2} Y^{2,*}_{i,\epsilon} Z^*_{\epsilon,\gamma} Y^{3,*}_{b,\gamma} Y^{4,*}_{j,\gamma} {}^2D^{a,i,b,j} {}^2T_{c,i,a,k} V_{b,j,k,c} \quad (691)$$

Factorized expression

$$\tau^0_{\gamma,\alpha,w} = \sum_{a \in V} {}^2D^3_{a,w} W^1_{a,\alpha} Y^{3,*}_{a,\gamma} \quad (3r_D r_T r_V N_v) \quad (692)$$

$$\tau^1_{\gamma,\alpha} = \sum_{a \in V} W^2_{a,\alpha} Y^3_{a,\gamma} \quad (2r_T r_V N_v) \quad (693)$$

$$\tau^2_{\gamma,\alpha,i} = \sum_{\delta \in A} Z_{\gamma,\delta} Y^4_{i,\delta} \tau^1_{\delta,\alpha} \quad (3r_T^2 r_V N_o) \quad (694)$$

$$\tau^3_{\gamma,\delta,\alpha,w} = \sum_{i \in O} {}^2D^4_{i,w} Y^{4,*}_{i,\delta} \tau^0_{\delta,\alpha,w} \tau^2_{\gamma,\alpha,i} \quad (4r_D r_T^2 r_V N_o) \quad (695)$$

$$\tau^4_{\alpha,i,j} = \sum_{\beta \in B} X_{\alpha,\beta} W^3_{i,\beta} W^4_{j,\beta} \quad (3r_V^2 N_o^2) \quad (696)$$

$$\tau^5_{\gamma,\alpha,i} = \sum_{j \in O} Y^2_{j,\gamma} \tau^4_{\alpha,j,i} \quad (2r_T r_V N_o^2) \quad (697)$$

$$\tau^6_{\gamma,\delta,w,i} = \sum_{\alpha \in B} \tau^5_{\gamma,\alpha,i} \tau^3_{\gamma,\delta,\alpha,w} \quad (2r_D r_T^2 r_V N_o) \quad (698)$$

$$\tau^7_{\gamma,\delta,w} = \sum_{\epsilon \in A} \sum_{i \in O} {}^2D^2_{i,w} Y^{2,*}_{i,\delta} Z^*_{\delta,\epsilon} \tau^6_{\gamma,\epsilon,w,i} \quad (4r_D r_T^3 N_o) \quad (699)$$

$${}^{21}R_{a,\gamma} \leftarrow - \sum_{\delta \in A} \sum_{w \in D} \frac{1}{2} {}^2D^1_{a,w} Y^1_{a,\delta} \tau^7_{\delta,\gamma,w} \quad (3r_D r_T^2 N_v) \quad (700)$$

Raw expression

$${}^{21}R_{a,\epsilon} \leftarrow - \sum_{\gamma \in A} \sum_{i \in O} \sum_{j \in O} \sum_{k \in O} \sum_{b \in V} \sum_{c \in V} \frac{1}{2} Y^{2,*}_{i,\epsilon} Z^*_{\epsilon,\gamma} Y^{3,*}_{b,\gamma} Y^{4,*}_{j,\gamma} {}^2D^{a,i,b,j} T_{c,i,b,k} V_{a,c,k,j} \quad (701)$$

Factorized expression

$$\tau^0_{\gamma,\alpha,w} = \sum_{a \in V} {}^2D^3_{a,w} W^1_{a,\alpha} Y^{3,*}_{a,\gamma} \quad (3r_D r_T r_V N_v) \quad (702)$$

$$\tau^1_{\gamma,\alpha} = \sum_{a \in V} W^2_{a,\alpha} Y^1_{a,\gamma} \quad (2r_T r_V N_v) \quad (703)$$

$$\tau^2_{\gamma,\alpha,i} = \sum_{\delta \in A} Y^2_{i,\delta} Z_{\delta,\gamma} \tau^1_{\delta,\alpha} \quad (3r_T^2 r_V N_o) \quad (704)$$

$$\tau^3_{\gamma,\delta,\alpha,w} = \sum_{i \in O} {}^2D^4_{i,w} Y^{4,*}_{i,\delta} \tau^0_{\delta,\alpha,w} \tau^2_{\gamma,\alpha,i} \quad (4r_D r_T^2 r_V N_o) \quad (705)$$

$$\tau^4_{\alpha,i,j} = \sum_{\beta \in B} X_{\alpha,\beta} W^3_{i,\beta} W^4_{j,\beta} \quad (3r_V^2 N_o^2) \quad (706)$$

$$\tau^5_{\gamma,\alpha,i} = \sum_{j \in O} Y^4_{j,\gamma} \tau^4_{\alpha,j,i} \quad (2r_T r_V N_o^2) \quad (707)$$

$$\tau^6_{\gamma,\delta,w,i} = \sum_{\alpha \in B} \tau^5_{\gamma,\alpha,i} \tau^3_{\gamma,\delta,\alpha,w} \quad (2r_D r_T^2 r_V N_o) \quad (708)$$

$$\tau^7_{\gamma,\delta,w} = \sum_{\epsilon \in A} \sum_{i \in O} {}^2D^2_{i,w} Y^{2,*}_{i,\delta} Z^*_{\delta,\epsilon} \tau^6_{\gamma,\epsilon,w,i} \quad (4r_D r_T^3 N_o) \quad (709)$$

$${}^{21}R_{a,\gamma} \leftarrow - \sum_{\delta \in A} \sum_{w \in D} \frac{1}{2} {}^2D^1_{a,w} Y^3_{a,\delta} \tau^7_{\delta,\gamma,w} \quad (3r_D r_T^2 N_v) \quad (710)$$

Raw expression

$${}^{21}R_{a,\epsilon} \leftarrow - \sum_{\gamma \in A} \sum_{i \in O} \sum_{j \in O} \sum_{k \in O} \sum_{b \in V} \sum_{c \in V} \frac{1}{2} Y^{2,*}_{i,\epsilon} Z^*_{\epsilon,\gamma} Y^{3,*}_{b,\gamma} Y^{4,*}_{j,\gamma} {}^2D^{a,i,b,j} T_{c,j,a,k} V_{b,c,k,i} \quad (711)$$

Factorized expression

$$\tau^0_{\gamma,\delta,w} = \sum_{i \in O} {}^2D^2_{i,w} Y^2_{i,\gamma} Y^{2,*}_{i,\delta} \quad (3r_D r_T^2 N_o) \quad (712)$$

$$\tau^1_{\alpha,i,j} = \sum_{\beta \in B} X_{\alpha,\beta} W^3_{i,\beta} W^4_{j,\beta} \quad (3r_V^2 N_o^2) \quad (713)$$

$$\tau^2_{\gamma,\alpha,i} = \sum_{j \in O} Y^4_{j,\gamma} \tau^1_{\alpha,j,i} \quad (2r_T r_V N_o^2) \quad (714)$$

$$\tau^3_{\gamma,\alpha} = \sum_{a \in V} W^2_{a,\alpha} Y^3_{a,\gamma} \quad (2r_T r_V N_v) \quad (715)$$

$$\tau^4_{\gamma,i,a} = \sum_{\alpha \in B} W^1_{a,\alpha} \tau^3_{\gamma,\alpha} \tau^2_{\gamma,\alpha,i} \quad (3r_T r_V N_o N_v) \quad (716)$$

$$\tau^5_{\gamma,\delta,w} = \sum_{i \in O} \sum_{a \in V} {}^2D^3_{a,w} {}^2D^4_{i,w} Y^{3,*}_{a,\delta} Y^{4,*}_{i,\delta} \tau^4_{\gamma,i,a} \quad (5r_D r_T^2 N_o N_v) \quad (717)$$

$$= \sum_{\delta \in A} \sum_{w \in D} \frac{1}{2} {}^2D^1_{a,w} Y^3_{a,\delta} \tau^0_{\delta,\gamma,w} \tau^7_{\delta,\gamma,w} \quad (4r_D r_T^2 N_v) \quad (730)$$

$$\tau^6_{\gamma,\delta,w} = \sum_{\epsilon \in A} Z^*_{\delta,\epsilon} \tau^5_{\gamma,\epsilon,w} \quad (2r_D r_T^3) \quad (718)$$

$$\tau^7_{\gamma,\delta,w} = \sum_{\epsilon \in A} Z_{\gamma,\epsilon} \tau^6_{\epsilon,\delta,w} \quad (2r_D r_T^3) \quad (719)$$

Raw expression

$${}^{21}R_{a,\epsilon} \leftarrow - \sum_{\gamma \in A} \sum_{i \in O} \sum_{j \in O} \sum_{k \in O} \sum_{b \in V} \sum_{c \in V} \frac{1}{2} Y^{2,*}_{i,\epsilon} Z^*_{\epsilon,\gamma} Y^{3,*}_{b,\gamma} Y^{4,*}_{j,\gamma} {}^2D^{a,i,b,j} {}^2T_{c,k,a,i} V_{b,c,k,j} \quad (731)$$

Factorized expression

$${}^{21}R_{a,\gamma} \leftarrow - \sum_{\delta \in A} \sum_{w \in D} \frac{1}{2} {}^2D^1_{a,w} Y^1_{a,\delta} \tau^0_{\delta,\gamma,w} \tau^7_{\delta,\gamma,w} \quad (4r_D r_T^2 N_v) \quad (720)$$

$$\tau^0_{\gamma,\alpha} = \sum_{i \in O} W^3_{i,\alpha} Y^2_{i,\gamma} \quad (2r_T r_V N_o) \quad (732)$$

Raw expression

$${}^{21}R_{a,\epsilon} \leftarrow - \sum_{\gamma \in A} \sum_{i \in O} \sum_{j \in O} \sum_{k \in O} \sum_{b \in V} \sum_{c \in V} \frac{1}{2} Y^{2,*}_{i,\epsilon} Z^*_{\epsilon,\gamma} Y^{3,*}_{b,\gamma} Y^{4,*}_{j,\gamma} {}^2D^{a,i,b,j} {}^2T_{c,j,b,k} V_{a,i,k,c} \quad (721)$$

$$\tau^1_{\gamma,\alpha} = \sum_{a \in V} W^4_{a,\alpha} Y^3_{a,\gamma} \quad (2r_T r_V N_v) \quad (733)$$

$$\tau^2_{\gamma,\alpha,i} = \sum_{\delta \in A} Z_{\gamma,\delta} Y^4_{i,\delta} \tau^1_{\delta,\alpha} \quad (3r_T^2 r_V N_o) \quad (734)$$

Factorized expression

$$\tau^0_{\gamma,\delta,w} = \sum_{i \in O} {}^2D^2_{i,w} Y^4_{i,\gamma} Y^{2,*}_{i,\delta} \quad (3r_D r_T^2 N_o) \quad (722)$$

$$\tau^3_{\gamma,\alpha,w} = \sum_{a \in V} {}^2D^3_{a,w} W^1_{a,\alpha} Y^{3,*}_{a,\gamma} \quad (3r_D r_T r_V N_v) \quad (735)$$

$$\tau^1_{\alpha,i,j} = \sum_{\beta \in B} X_{\alpha,\beta} W^3_{i,\beta} W^4_{j,\beta} \quad (3r_V^2 N_o^2) \quad (723)$$

$$\tau^4_{\gamma,\alpha,w} = \sum_{i \in O} {}^2D^4_{i,w} W^2_{i,\alpha} Y^{4,*}_{i,\gamma} \quad (3r_D r_T r_V N_o) \quad (736)$$

$$\tau^2_{\gamma,\alpha,i} = \sum_{j \in O} Y^2_{j,\gamma} \tau^1_{\alpha,j,i} \quad (2r_T r_V N_o^2) \quad (724)$$

$$\tau^5_{\gamma,\alpha,w} = \sum_{\beta \in B} X_{\beta,\alpha} \tau^3_{\gamma,\beta,w} \tau^4_{\gamma,\beta,w} \quad (3r_D r_T r_V^2) \quad (737)$$

$$\tau^3_{\gamma,\alpha} = \sum_{a \in V} W^2_{a,\alpha} Y^1_{a,\gamma} \quad (2r_T r_V N_v) \quad (725)$$

$$\tau^6_{\gamma,\alpha,w} = \sum_{\delta \in A} Z^*_{\gamma,\delta} \tau^5_{\delta,\alpha,w} \quad (2r_D r_T^2 r_V) \quad (738)$$

$$\tau^4_{\gamma,i,a} = \sum_{\alpha \in B} W^1_{a,\alpha} \tau^3_{\gamma,\alpha} \tau^2_{\gamma,\alpha,i} \quad (3r_T r_V N_o N_v) \quad (726)$$

$$\tau^7_{\gamma,\delta,w,i} = \sum_{\alpha \in B} \tau^0_{\gamma,\alpha} \tau^2_{\gamma,\alpha,i} \tau^6_{\delta,\alpha,w} \quad (3r_D r_T^2 r_V N_o) \quad (739)$$

$$\tau^5_{\gamma,\delta,w} = \sum_{i \in O} \sum_{a \in V} {}^2D^3_{a,w} {}^2D^4_{i,w} Y^{3,*}_{a,\delta} Y^{4,*}_{i,\delta} \tau^4_{\gamma,i,a} \quad (5r_D r_T^2 N_o N_v) \quad (727)$$

$$\tau^8_{\gamma,\delta,w} = \sum_{i \in O} {}^2D^2_{i,w} Y^{2,*}_{i,\delta} \tau^7_{\gamma,\delta,w,i} \quad (3r_D r_T^2 N_o) \quad (740)$$

$$\tau^6_{\gamma,\delta,w} = \sum_{\epsilon \in A} Z^*_{\delta,\epsilon} \tau^5_{\gamma,\epsilon,w} \quad (2r_D r_T^3) \quad (728)$$

$$\tau^7_{\gamma,\delta,w} = \sum_{\epsilon \in A} Z_{\epsilon,\gamma} \tau^6_{\epsilon,\delta,w} \quad (2r_D r_T^3) \quad (729)$$

$${}^{21}R_{a,\gamma} \leftarrow - \sum_{\delta \in A} \sum_{w \in D} \frac{1}{2} {}^2D^1_{a,w} Y^1_{a,\delta} \tau^8_{\delta,\gamma,w} \quad (3r_D r_T^2 N_v) \quad (741)$$

Raw expression

$${}^{21}R_{a,\epsilon} \leftarrow - \sum_{\gamma \in A} \sum_{i \in O} \sum_{j \in O} \sum_{k \in O} \sum_{b \in V} \sum_{c \in V} \frac{1}{2} Y^{2,*}_{i,\epsilon} Z^{*}_{\epsilon,\gamma} Y^{3,*}_{b,\gamma} Y^{4,*}_{j,\gamma} {}^2D^{a,i,b,j} {}^2T_{c,k,b,j} V_{a,c,k,i} \quad (742)$$

Factorized expression

$$\tau^0_{\gamma,\alpha} = \sum_{a \in V} W^4_{a,\alpha} Y^1_{a,\gamma} \quad (2r_T r_V N_v) \quad (743)$$

$$\tau^1_{\gamma,\alpha,i} = \sum_{\delta \in A} Y^2_{i,\delta} Z_{\delta,\gamma} \tau^0_{\delta,\alpha} \quad (3r_T^2 r_V N_o) \quad (744)$$

$$\tau^2_{\gamma,\alpha} = \sum_{i \in O} W^3_{i,\alpha} Y^4_{i,\gamma} \quad (2r_T r_V N_o) \quad (745)$$

$$\tau^3_{\gamma,\alpha,w} = \sum_{a \in V} {}^2D^3_{a,w} W^1_{a,\alpha} Y^{3,*}_{a,\gamma} \quad (3r_D r_T r_V N_v) \quad (746)$$

$$\tau^4_{\gamma,\alpha,w} = \sum_{i \in O} {}^2D^4_{i,w} W^2_{i,\alpha} Y^{4,*}_{i,\gamma} \quad (3r_D r_T r_V N_o) \quad (747)$$

$$\tau^5_{\gamma,\alpha,w} = \sum_{\beta \in B} X_{\beta,\alpha} \tau^3_{\gamma,\beta,w} \tau^4_{\gamma,\beta,w} \quad (3r_D r_T r_V^2) \quad (748)$$

$$\tau^6_{\gamma,\alpha,w} = \sum_{\delta \in A} Z^*_{\gamma,\delta} \tau^5_{\delta,\alpha,w} \quad (2r_D r_T^2 r_V) \quad (749)$$

$$\tau^7_{\gamma,\delta,w,i} = \sum_{\alpha \in B} \tau^2_{\gamma,\alpha} \tau^1_{\gamma,\alpha,i} \tau^6_{\delta,\alpha,w} \quad (3r_D r_T^2 r_V N_o) \quad (750)$$

$$\tau^8_{\gamma,\delta,w} = \sum_{i \in O} {}^2D^2_{i,w} Y^{2,*}_{i,\delta} \tau^7_{\gamma,\delta,w,i} \quad (3r_D r_T^2 N_o) \quad (751)$$

$${}^{21}R_{a,\gamma} \leftarrow - \sum_{\delta \in A} \sum_{w \in D} \frac{1}{2} {}^2D^1_{a,w} Y^3_{a,\delta} \tau^8_{\delta,\gamma,w} \quad (3r_D r_T^2 N_v) \quad (752)$$

Raw expression

$${}^{21}R_{a,\epsilon} \leftarrow \sum_{\gamma \in A} \sum_{i \in O} \sum_{j \in O} \sum_{b \in V} \sum_{c \in V} \sum_{d \in V} \frac{1}{2} Y^{2,*}_{i,\epsilon} Z^{*}_{\epsilon,\gamma} Y^{3,*}_{b,\gamma} Y^{4,*}_{j,\gamma} {}^2D^{a,i,b,j} {}^2T_{c,i,d,j} V_{a,c,b,d} \quad (753)$$

Factorized expression

$$\tau^0_{\gamma,\delta,w} = \sum_{a \in V} {}^2D^3_{a,w} Y^3_{a,\gamma} Y^{3,*}_{a,\delta} \quad (3r_D r_T^2 N_v) \quad (754)$$

$$\tau^1_{\gamma,i} = \sum_{j \in O} Y^4_{j,\gamma} f_{j,i} \quad (2r_T N_o^2) \quad (755)$$

$$\tau^2_{\gamma,\delta,w} = \sum_{i \in O} {}^2D^4_{i,w} Y^{4,*}_{i,\delta} \tau^1_{\gamma,i} \quad (3r_D r_T^2 N_o) \quad (756)$$

$$\tau^3_{\gamma,\delta,w} = \sum_{\epsilon \in A} Z^*_{\delta,\epsilon} \tau^0_{\gamma,\epsilon,w} \tau^2_{\gamma,\epsilon,w} \quad (3r_D r_T^3) \quad (757)$$

$$\tau^4_{\gamma,\delta,w} = \sum_{\epsilon \in A} Z_{\gamma,\epsilon} \tau^3_{\epsilon,\delta,w} \quad (2r_D r_T^3) \quad (758)$$

$$\tau^5_{\gamma,\delta,w} = \sum_{i \in O} {}^2D^2_{i,w} Y^2_{i,\gamma} Y^{2,*}_{i,\delta} \quad (3r_D r_T^2 N_o) \quad (759)$$

$${}^{21}R_{a,\gamma} \leftarrow - \sum_{\delta \in A} \sum_{w \in D} \frac{1}{2} {}^2D^1_{a,w} Y^1_{a,\delta} \tau^4_{\delta,\gamma,w} \tau^5_{\delta,\gamma,w} \quad (4r_D r_T^2 N_v) \quad (760)$$

Raw expression

$${}^{21}R_{a,\epsilon} \leftarrow \sum_{\gamma \in A} \sum_{i \in O} \sum_{j \in O} \sum_{b \in V} \sum_{c \in V} \sum_{d \in V} \frac{1}{2} Y^{2,*}_{i,\epsilon} Z^{*}_{\epsilon,\gamma} Y^{3,*}_{b,\gamma} Y^{4,*}_{j,\gamma} {}^2D^{a,i,b,j} {}^2T_{c,j,d,i} V_{a,d,b,c} \quad (761)$$

Factorized expression

$$\tau^0_{\gamma,i} = \sum_{j \in O} Y^2_{j,\gamma} f_{j,i} \quad (2r_T N_o^2) \quad (762)$$

$$\tau^1_{\gamma,\delta,w} = \sum_{i \in O} {}^2D^2_{i,w} Y^{2,*}_{i,\delta} \tau^0_{\gamma,i} \quad (3r_D r_T^2 N_o) \quad (763)$$

$$\tau^2_{\gamma,\delta,w} = \sum_{a \in V} {}^2D^3_{a,w} Y^3_{a,\gamma} Y^{3,*}_{a,\delta} \quad (3r_D r_T^2 N_v) \quad (764)$$

$$\tau^3_{\gamma,\delta,w} = \sum_{i \in O} {}^2D^4_{i,w} Y^4_{i,\gamma} Y^{4,*}_{i,\delta} \quad (3r_D r_T^2 N_o) \quad (765)$$

$$\tau^4_{\gamma,\delta,w} = \sum_{\epsilon \in A} Z^*_{\delta,\epsilon} \tau^2_{\gamma,\epsilon,w} \tau^3_{\gamma,\epsilon,w} \quad (3r_D r_T^3) \quad (766)$$

$$\tau_{\gamma,\delta,w}^5 = \sum_{\epsilon \in A} Z_{\gamma,\epsilon} \tau_{\epsilon,\delta,w}^4 \quad (2r_D r_T^3) \quad (767)$$

$$\tau_{\gamma,i}^1 = \sum_{j \in O} Y_{j,\gamma}^2 f_{j,i} \quad (2r_T N_o^2) \quad (779)$$

$${}^{21}R_{a,\gamma} \leftarrow - \sum_{\delta \in A} \sum_{w \in D} \frac{1}{2} {}^2D_{a,w}^1 Y_{a,\delta}^1 \tau_{\delta,\gamma,w}^1 \tau_{\delta,\gamma,w}^5 \quad (4r_D r_T^2 N_v) \quad \tau_{\gamma,\delta,w}^2 = \sum_{i \in O} {}^2D_{i,w}^4 Y_{i,\delta}^{4,*} \tau_{\gamma,i}^1 \quad (3r_D r_T^2 N_o) \quad (780)$$

Raw expression

$$\tau_{\gamma,\delta,w}^3 = \sum_{\epsilon \in A} Z_{\delta,\epsilon}^* \tau_{\gamma,\epsilon,w}^0 \tau_{\gamma,\epsilon,w}^2 \quad (3r_D r_T^3) \quad (781)$$

$${}^{21}R_{a,\epsilon} \leftarrow \sum_{\gamma \in A} \sum_{i \in O} \sum_{j \in O} \sum_{b \in V} \sum_{c \in V} \frac{1}{2} Y_{i,\epsilon}^{2,*} Z_{\epsilon,\gamma}^* Y_{b,\gamma}^{3,*} Y_{j,\gamma}^{4,*} f_{a,c} {}^2D_{a,i,b,j} {}^2T_{b,j,c,i} \quad (769)$$

$$\tau_{\gamma,\delta,w}^4 = \sum_{\epsilon \in A} Z_{\epsilon,\gamma} \tau_{\epsilon,\delta,w}^3 \quad (2r_D r_T^3) \quad (782)$$

Factorized expression

$$\tau_{\gamma,\delta,w}^5 = \sum_{i \in O} {}^2D_{i,w}^2 Y_{i,\gamma}^4 Y_{i,\delta}^{2,*} \quad (3r_D r_T^2 N_o) \quad (783)$$

$$\tau_{\gamma,i}^0 = \sum_{j \in O} Y_{j,\gamma}^4 f_{j,i} \quad (2r_T N_o^2) \quad (770)$$

$${}^{21}R_{a,\gamma} \leftarrow - \sum_{\delta \in A} \sum_{w \in D} \frac{1}{2} {}^2D_{a,w}^1 Y_{a,\delta}^3 \tau_{\delta,\gamma,w}^4 \tau_{\delta,\gamma,w}^5 \quad (4r_D r_T^2 N_v) \quad (784)$$

Raw expression

$$\tau_{\gamma,\delta,w}^2 = \sum_{a \in V} {}^2D_{a,w}^3 Y_{a,\gamma}^1 Y_{a,\delta}^{3,*} \quad (3r_D r_T^2 N_v) \quad (772)$$

$${}^{21}R_{a,\epsilon} \leftarrow \sum_{\gamma \in A} \sum_{i \in O} \sum_{j \in O} \sum_{b \in V} \sum_{c \in V} \frac{1}{2} Y_{i,\epsilon}^{2,*} Z_{\epsilon,\gamma}^* Y_{b,\gamma}^{3,*} Y_{j,\gamma}^{4,*} f_{b,c} {}^2D_{a,i,b,j} {}^2T_{a,i,c,j} \quad (785)$$

$$\tau_{\gamma,\delta,w}^3 = \sum_{i \in O} {}^2D_{i,w}^4 Y_{i,\gamma}^2 Y_{i,\delta}^{4,*} \quad (3r_D r_T^2 N_o) \quad (773)$$

Factorized expression

$$\tau_{\gamma,\delta,w}^4 = \sum_{\epsilon \in A} Z_{\delta,\epsilon}^* \tau_{\gamma,\epsilon,w}^2 \tau_{\gamma,\epsilon,w}^3 \quad (3r_D r_T^3) \quad (774)$$

$$\tau_{\gamma,\alpha,w}^0 = \sum_{i \in O} {}^2D_{i,w}^4 W_{i,\alpha}^4 Y_{i,\gamma}^{4,*} \quad (3r_D r_T r_V N_o) \quad (786)$$

$$\tau_{\gamma,\delta,w}^5 = \sum_{\epsilon \in A} Z_{\epsilon,\gamma} \tau_{\epsilon,\delta,w}^4 \quad (2r_D r_T^3) \quad (775)$$

$$\tau_{\gamma,\delta,w}^1 = \sum_{a \in V} {}^2D_{a,w}^3 Y_{a,\gamma}^3 Y_{a,\delta}^{3,*} \quad (3r_D r_T^2 N_v) \quad (787)$$

$${}^{21}R_{a,\gamma} \leftarrow - \sum_{\delta \in A} \sum_{w \in D} \frac{1}{2} {}^2D_{a,w}^1 Y_{a,\delta}^3 \tau_{\delta,\gamma,w}^1 \tau_{\delta,\gamma,w}^5 \quad (4r_D r_T^2 N_v) \quad \tau_{\gamma,\delta,w,i}^2 = \sum_{\epsilon \in A} Z_{\gamma,\epsilon} Y_{i,\epsilon}^4 \tau_{\epsilon,\delta,w}^1 \quad (3r_D r_T^3 N_o) \quad (788)$$

Raw expression

$$\tau_{\gamma,\delta,\alpha,w}^3 = \sum_{i \in O} W_{i,\alpha}^3 \tau_{\delta,\alpha,w}^0 \tau_{\gamma,\delta,w,i}^2 \quad (3r_D r_T^2 r_V N_o) \quad (789)$$

$${}^{21}R_{a,\epsilon} \leftarrow \sum_{\gamma \in A} \sum_{i \in O} \sum_{j \in O} \sum_{b \in V} \sum_{c \in V} \frac{1}{2} Y_{i,\epsilon}^{2,*} Z_{\epsilon,\gamma}^* Y_{b,\gamma}^{3,*} Y_{j,\gamma}^{4,*} f_{a,c} {}^2D_{a,i,b,j} {}^2T_{c,i,b,j} \quad (777)$$

$$\tau_{\alpha,i,j}^4 = \sum_{\beta \in B} W_{i,\beta}^1 W_{j,\beta}^2 X_{\beta,\alpha} \quad (3r_V^2 N_o^2) \quad (790)$$

Factorized expression

$$\tau_{\gamma,\delta,w}^0 = \sum_{a \in V} {}^2D_{a,w}^3 Y_{a,\gamma}^1 Y_{a,\delta}^{3,*} \quad (3r_D r_T^2 N_v) \quad (778)$$

$$\tau_{\gamma,\alpha,i}^5 = \sum_{j \in O} Y_{j,\gamma}^2 \tau_{\alpha,j,i}^4 \quad (2r_T r_V N_o^2) \quad (791)$$



$$\tau_{\gamma,\delta,w,i}^6 = \sum_{\alpha \in B} \tau_{\gamma,\alpha,i}^5 \tau_{\gamma,\delta,\alpha,w}^3 \quad (2r_D r_T^2 r_V N_o) \quad (792)$$

$$\tau_{\gamma,\delta,w}^7 = \sum_{\epsilon \in A} \sum_{i \in O} {}^2D_{i,w}^2 Y_{i,\delta}^{2,*} Z_{\delta,\epsilon}^* \tau_{\gamma,\epsilon,w,i}^6 \quad (4r_D r_T^3 N_o) \quad (793)$$

$${}^{21}R_{a,\gamma} \leftarrow \sum_{\delta \in A} \sum_{w \in D} \frac{1}{2} {}^2D_{a,w}^1 Y_{a,\delta}^1 \tau_{\delta,\gamma,w}^7 \quad (3r_D r_T^2 N_v) \quad (794)$$

Raw expression

$${}^{21}R_{a,\epsilon} \leftarrow \sum_{\gamma \in A} \sum_{i \in O} \sum_{j \in O} \sum_{b \in V} \sum_{c \in V} \frac{1}{2} Y_{i,\epsilon}^{2,*} Z_{\epsilon,\gamma}^* Y_{b,\gamma}^{3,*} Y_{j,\gamma}^{4,*} f_{b,c} {}^2D_{c,j,a,i}^{a,i,b,j} {}^2T_{c,j,a,i} \quad (795)$$

Factorized expression

$$\tau_{\gamma,\alpha,w}^0 = \sum_{i \in O} {}^2D_{i,w}^4 W_{i,\alpha}^4 Y_{i,\gamma}^{4,*} \quad (3r_D r_T r_V N_o) \quad (796)$$

$$\tau_{\gamma,\delta,w}^1 = \sum_{a \in V} {}^2D_{a,w}^3 Y_{a,\gamma}^1 Y_{a,\delta}^{3,*} \quad (3r_D r_T^2 N_v) \quad (797)$$

$$\tau_{\gamma,\delta,w,i}^2 = \sum_{\epsilon \in A} Y_{i,\epsilon}^2 Z_{\epsilon,\gamma} \tau_{\epsilon,\delta,w}^1 \quad (3r_D r_T^3 N_o) \quad (798)$$

$$\tau_{\gamma,\delta,\alpha,w}^3 = \sum_{i \in O} W_{i,\alpha}^3 \tau_{\delta,\alpha,w}^0 \tau_{\gamma,\delta,w,i}^2 \quad (3r_D r_T^2 r_V N_o) \quad (799)$$

$$\tau_{\alpha,i,j}^4 = \sum_{\beta \in B} W_{i,\beta}^1 W_{j,\beta}^2 X_{\beta,\alpha} \quad (3r_V^2 N_o^2) \quad (800)$$

$$\tau_{\gamma,\alpha,i}^5 = \sum_{j \in O} Y_{j,\gamma}^4 \tau_{\alpha,j,i}^4 \quad (2r_T r_V N_o^2) \quad (801)$$

$$\tau_{\gamma,\delta,w,i}^6 = \sum_{\alpha \in B} \tau_{\gamma,\alpha,i}^5 \tau_{\gamma,\delta,\alpha,w}^3 \quad (2r_D r_T^2 r_V N_o) \quad (802)$$

$$\tau_{\gamma,\delta,w}^7 = \sum_{\epsilon \in A} \sum_{i \in O} {}^2D_{i,w}^2 Y_{i,\delta}^{2,*} Z_{\delta,\epsilon}^* \tau_{\gamma,\epsilon,w,i}^6 \quad (4r_D r_T^3 N_o) \quad (803)$$

$${}^{21}R_{a,\gamma} \leftarrow \sum_{\delta \in A} \sum_{w \in D} \frac{1}{2} {}^2D_{a,w}^1 Y_{a,\delta}^3 \tau_{\delta,\gamma,w}^7 \quad (3r_D r_T^2 N_v) \quad (804)$$

## E. Contributions from $(H^1 T^1 T^1 T)_c$

Raw expression

$${}^{21}R_{a,\epsilon} \leftarrow \sum_{\gamma \in A} \sum_{i \in O} \sum_{j \in O} \sum_{k \in O} \sum_{l \in O} \sum_{b \in V} \sum_{c \in V} {}^1T_{a,k} {}^1T_{b,l} {}^1T_{c,i} Y_{i,\epsilon}^{2,*} Z_{\epsilon,\gamma}^* Y_{b,\gamma}^{3,*} Y_{j,\gamma}^{4,*} {}^2D_{a,i,b,j} V_{k,c,l,j} \quad (805)$$

Factorized expression

$$\tau_{\alpha,i}^0 = \sum_{a \in V} {}^1T_{a,i} W_{a,\alpha}^4 \quad (2r_V N_o N_v) \quad (806)$$

$$\tau_{\gamma,\alpha,w}^1 = \sum_{i \in O} {}^2D_{i,w}^2 Y_{i,\gamma}^{2,*} \tau_{\alpha,i}^0 \quad (3r_D r_T r_V N_o) \quad (807)$$

$$\tau_{\alpha,i}^2 = \sum_{a \in V} {}^1T_{a,i} W_{a,\alpha}^2 \quad (2r_V N_o N_v) \quad (808)$$

$$\tau_{\gamma,\alpha,w}^3 = \sum_{i \in O} {}^2D_{i,w}^4 Y_{i,\gamma}^{4,*} \tau_{\alpha,i}^2 \quad (3r_D r_T r_V N_o) \quad (809)$$

$$\tau_{\gamma,\alpha,w}^4 = \sum_{a \in V} {}^2D_{a,w}^3 W_{a,\alpha}^1 Y_{a,\gamma}^{3,*} \quad (3r_D r_T r_V N_v) \quad (810)$$

$$\tau_{\gamma,\alpha,w}^5 = \sum_{\beta \in B} X_{\beta,\alpha} \tau_{\gamma,\beta,w}^3 \tau_{\gamma,\beta,w}^4 \quad (3r_D r_T r_V^2) \quad (811)$$

$$\tau_{\gamma,\alpha,w}^6 = \sum_{\delta \in A} Z_{\gamma,\delta}^* \tau_{\delta,\alpha,w}^5 \quad (2r_D r_T^2 r_V) \quad (812)$$

$$\tau_{\gamma,w,i}^7 = \sum_{\alpha \in B} W_{i,\alpha}^3 \tau_{\gamma,\alpha,w}^1 \tau_{\gamma,\alpha,w}^6 \quad (3r_D r_T r_V N_o) \quad (813)$$

$${}^{21}R_{a,\gamma} \leftarrow - \sum_{w \in D} \sum_{i \in O} {}^2D_{a,w}^1 {}^1T_{a,i} \tau_{\gamma,w,i}^7 \quad (3r_D r_T N_o N_v) \quad (814)$$

Raw expression

$${}^{21}R_{a,\epsilon} \leftarrow \sum_{\gamma \in A} \sum_{i \in O} \sum_{j \in O} \sum_{k \in O} \sum_{l \in O} \sum_{b \in V} \sum_{c \in V} {}^1T_{a,k} {}^1T_{b,l} {}^1T_{c,j} Y_{i,\epsilon}^{2,*} Z_{\epsilon,\gamma}^* Y_{b,\gamma}^{3,*} Y_{j,\gamma}^{4,*} {}^2D_{a,i,b,j} V_{k,i,l,c} \quad (815)$$

Factorized expression

$$\tau^0_{\alpha,i} = \sum_{a \in V} {}^1T_{a,i} W^2_{a,\alpha} \quad (2r_V N_o N_v) \quad (816)$$

$$\tau^1_{\gamma,\alpha,w} = \sum_{i \in O} {}^2D^2_{i,w} Y^{2,*}_{i,\gamma} \tau^0_{\alpha,i} \quad (3r_D r_T r_V N_o) \quad (817)$$

$$\tau^2_{\alpha,i} = \sum_{a \in V} {}^1T_{a,i} W^4_{a,\alpha} \quad (2r_V N_o N_v) \quad (818)$$

$$\tau^3_{\gamma,\alpha,w} = \sum_{i \in O} {}^2D^4_{i,w} Y^{4,*}_{i,\gamma} \tau^2_{\alpha,i} \quad (3r_D r_T r_V N_o) \quad (819)$$

$$\tau^4_{\gamma,w,i} = \sum_{a \in V} {}^2D^3_{a,w} {}^1T_{a,i} Y^{3,*}_{a,\gamma} \quad (3r_D r_T N_o N_v) \quad (820)$$

$$\tau^5_{\gamma,\alpha,w} = \sum_{i \in O} W^3_{i,\alpha} \tau^4_{\gamma,w,i} \quad (2r_D r_T r_V N_o) \quad (821)$$

$$\tau^6_{\gamma,\alpha,w} = \sum_{\beta \in B} X_{\alpha,\beta} \tau^3_{\gamma,\beta,w} \tau^5_{\gamma,\beta,w} \quad (3r_D r_T r_V^2) \quad (822)$$

$$\tau^7_{\gamma,\alpha,w} = \sum_{\delta \in A} Z^*_{\gamma,\delta} \tau^6_{\delta,\alpha,w} \quad (2r_D r_T^2 r_V) \quad (823)$$

$$\tau^8_{\gamma,w,a} = \sum_{\alpha \in B} W^1_{a,\alpha} \tau^1_{\gamma,\alpha,w} \tau^7_{\gamma,\alpha,w} \quad (3r_D r_T r_V N_v) \quad (824)$$

$${}^{21}R_{a,\gamma} \leftarrow - \sum_{w \in D} {}^2D^1_{a,w} \tau^8_{\gamma,w,a} \quad (2r_D r_T N_v) \quad (825)$$

Raw expression

$${}^{21}R_{a,\epsilon} \leftarrow - \sum_{\gamma \in A} \sum_{i \in O} \sum_{j \in O} \sum_{k \in O} \sum_{b \in V} \sum_{c \in V} \sum_{d \in V} {}^1T_{a,k} {}^1T_{c,i} {}^1T_{d,j} Y^{2,*}_{i,\epsilon} Z^*_{\epsilon,\gamma} Y^{3,*}_{b,\gamma} Y^{4,*}_{j,\gamma} {}^2D^{a,i,b,j} V_{b,d,k,c} \quad (826)$$

Factorized expression

$$\tau^0_{\alpha,i} = \sum_{a \in V} {}^1T_{a,i} W^2_{a,\alpha} \quad (2r_V N_o N_v) \quad (827)$$

$$\tau^1_{\gamma,\alpha,w} = \sum_{i \in O} {}^2D^2_{i,w} Y^{2,*}_{i,\gamma} \tau^0_{\alpha,i} \quad (3r_D r_T r_V N_o) \quad (828)$$

$$\tau^2_{\gamma,w,i} = \sum_{a \in V} {}^2D^3_{a,w} {}^1T_{a,i} Y^{3,*}_{a,\gamma} \quad (3r_D r_T N_o N_v) \quad (829)$$

$$\tau^3_{\gamma,\alpha,w} = \sum_{i \in O} W^3_{i,\alpha} \tau^2_{\gamma,w,i} \quad (2r_D r_T r_V N_o) \quad (830)$$

$$\tau^4_{\gamma,\alpha,w} = \sum_{i \in O} {}^2D^4_{i,w} W^4_{i,\alpha} Y^{4,*}_{i,\gamma} \quad (3r_D r_T r_V N_o) \quad (831)$$

$$\tau^5_{\gamma,\alpha,w} = \sum_{\beta \in B} X_{\alpha,\beta} \tau^3_{\gamma,\beta,w} \tau^4_{\gamma,\beta,w} \quad (3r_D r_T r_V^2) \quad (832)$$

$$\tau^6_{\gamma,\alpha,w} = \sum_{\delta \in A} Z^*_{\gamma,\delta} \tau^5_{\delta,\alpha,w} \quad (2r_D r_T^2 r_V) \quad (833)$$

$$\tau^7_{\gamma,w,i} = \sum_{\alpha \in B} W^1_{i,\alpha} \tau^1_{\gamma,\alpha,w} \tau^6_{\gamma,\alpha,w} \quad (3r_D r_T r_V N_o) \quad (834)$$

$${}^{21}R_{a,\gamma} \leftarrow \sum_{w \in D} \sum_{i \in O} {}^2D^1_{a,w} {}^1T_{a,i} \tau^7_{\gamma,w,i} \quad (3r_D r_T N_o N_v) \quad (835)$$

Raw expression

$${}^{21}R_{a,\epsilon} \leftarrow - \sum_{\gamma \in A} \sum_{i \in O} \sum_{j \in O} \sum_{k \in O} \sum_{b \in V} \sum_{c \in V} \sum_{d \in V} {}^1T_{b,k} {}^1T_{c,i} {}^1T_{d,j} Y^{2,*}_{i,\epsilon} Z^*_{\epsilon,\gamma} Y^{3,*}_{b,\gamma} Y^{4,*}_{j,\gamma} {}^2D^{a,i,b,j} V_{a,c,k,d} \quad (836)$$

Factorized expression

$$\tau^0_{\gamma,\alpha,w} = \sum_{i \in O} {}^2D^2_{i,w} W^2_{i,\alpha} Y^{2,*}_{i,\gamma} \quad (3r_D r_T r_V N_o) \quad (837)$$

$$\tau^1_{\alpha,i} = \sum_{a \in V} {}^1T_{a,i} W^4_{a,\alpha} \quad (2r_V N_o N_v) \quad (838)$$

$$\tau^2_{\gamma,\alpha,w} = \sum_{i \in O} {}^2D^4_{i,w} Y^{4,*}_{i,\gamma} \tau^1_{\alpha,i} \quad (3r_D r_T r_V N_o) \quad (839)$$

$$\tau^3_{\gamma,w,i} = \sum_{a \in V} {}^2D^3_{a,w} {}^1T_{a,i} Y^{3,*}_{a,\gamma} \quad (3r_D r_T N_o N_v) \quad (840)$$

$$\tau^4_{\gamma,\alpha,w} = \sum_{i \in O} W^3_{i,\alpha} \tau^3_{\gamma,w,i} \quad (2r_D r_T r_V N_o) \quad (841)$$

$$\tau^5_{\gamma,\alpha,w} = \sum_{\beta \in B} X_{\alpha,\beta} \tau^2_{\gamma,\beta,w} \tau^4_{\gamma,\beta,w} \quad (3r_D r_T r_V^2) \quad (842)$$

$$\tau^6_{\gamma,\alpha,w} = \sum_{\delta \in A} Z^*_{\gamma,\delta} \tau^5_{\delta,\alpha,w} \quad (2r_D r_T^2 r_V) \quad (843)$$

$$\tau^7_{\gamma,w,i} = \sum_{\alpha \in B} W^1_{i,\alpha} \tau^0_{\gamma,\alpha,w} \tau^6_{\gamma,\alpha,w} \quad (3r_D r_T r_V N_o) \quad (844)$$

$${}^{21}R_{a,\gamma} \leftarrow \sum_{w \in D} \sum_{i \in O} {}^2D^1_{a,w} {}^1T_{a,i} \tau^7_{\gamma,w,i} \quad (3r_D r_T N_o N_v) \quad (845)$$

#### F. Contributions from $(H^1 T^2 T)_c$

Raw expression

$${}^{21}R_{a,\epsilon} \leftarrow - \sum_{\gamma \in A} \sum_{i \in O} \sum_{j \in O} \sum_{k \in O} \sum_{b \in V} \sum_{c \in V} \frac{1}{2} {}^1T_{a,k} Y^{2,*}_{i,\epsilon} Z^*_{\epsilon,\gamma} Y^{3,*}_{b,\gamma} Y^{4,*}_{j,\gamma} f_{k,c} {}^2D^{a,i,b,j} {}^2T_{b,j,c,i} \quad (846)$$

Factorized expression

$$\tau^0_{\gamma,\alpha} = \sum_{a \in V} W^4_{a,\alpha} Y^3_{a,\gamma} \quad (2r_T r_V N_v) \quad (847)$$

$$\tau^1_{\gamma,\alpha} = \sum_{i \in O} W^3_{i,\alpha} Y^4_{i,\gamma} \quad (2r_T r_V N_o) \quad (848)$$

$$\tau^2_{\gamma,\alpha} = \sum_{\beta \in B} X_{\alpha,\beta} \tau^0_{\gamma,\beta} \tau^1_{\gamma,\beta} \quad (3r_T r_V^2) \quad (849)$$

$$\tau^3_{\gamma,\alpha} = \sum_{\delta \in A} Z_{\gamma,\delta} \tau^2_{\delta,\alpha} \quad (2r_T^2 r_V) \quad (850)$$

$$\tau^4_{\gamma,\delta,w} = \sum_{a \in V} {}^2D^3_{a,w} Y^1_{a,\gamma} Y^{3,*}_{a,\delta} \quad (3r_D r_T^2 N_v) \quad (851)$$

$$\tau^5_{\gamma,\delta,w} = \sum_{i \in O} {}^2D^4_{i,w} Y^2_{i,\gamma} Y^{4,*}_{i,\delta} \quad (3r_D r_T^2 N_o) \quad (852)$$

$$\tau^6_{\gamma,\delta,w} = \sum_{\epsilon \in A} Z^*_{\delta,\epsilon} \tau^4_{\gamma,\epsilon,w} \tau^5_{\gamma,\epsilon,w} \quad (3r_D r_T^3) \quad (853)$$

$$\tau^7_{\gamma,\alpha,w} = \sum_{\delta \in A} \tau^3_{\delta,\alpha} \tau^6_{\delta,\gamma,w} \quad (2r_D r_T^2 r_V) \quad (854)$$

$$\tau^8_{\alpha,i} = \sum_{a \in V} {}^1T_{a,i} W^2_{a,\alpha} \quad (2r_V N_o N_v) \quad (855)$$

$$\tau^9_{\gamma,\alpha,w} = \sum_{i \in O} {}^2D^2_{i,w} Y^{2,*}_{i,\gamma} \tau^8_{\alpha,i} \quad (3r_D r_T r_V N_o) \quad (856)$$

$$\tau^{10}_{\gamma,w,a} = \sum_{\alpha \in B} W^1_{a,\alpha} \tau^7_{\gamma,\alpha,w} \tau^9_{\gamma,\alpha,w} \quad (3r_D r_T r_V N_v) \quad (857)$$

$${}^{21}R_{a,\gamma} \leftarrow \sum_{w \in D} {}^2D^1_{a,w} \tau^{10}_{\gamma,w,a} \quad (2r_D r_T N_v) \quad (858)$$

Raw expression

$${}^{21}R_{a,\epsilon} \leftarrow - \sum_{\gamma \in A} \sum_{i \in O} \sum_{j \in O} \sum_{k \in O} \sum_{b \in V} \sum_{c \in V} \frac{1}{2} {}^1T_{a,k} Y^{2,*}_{i,\epsilon} Z^*_{\epsilon,\gamma} Y^{3,*}_{b,\gamma} Y^{4,*}_{j,\gamma} f_{k,c} {}^2D^{a,i,b,j} {}^2T_{c,i,b,j} \quad (859)$$

Factorized expression

$$\tau^0_{\gamma,\delta,w} = \sum_{a \in V} {}^2D^3_{a,w} Y^3_{a,\gamma} Y^{3,*}_{a,\delta} \quad (3r_D r_T^2 N_v) \quad (860)$$

$$\tau^1_{\gamma,\delta,w} = \sum_{i \in O} {}^2D^4_{i,w} Y^4_{i,\gamma} Y^{4,*}_{i,\delta} \quad (3r_D r_T^2 N_o) \quad (861)$$

$$\tau^2_{\gamma,\delta,w} = \sum_{\epsilon \in A} Z^*_{\delta,\epsilon} \tau^0_{\gamma,\epsilon,w} \tau^1_{\gamma,\epsilon,w} \quad (3r_D r_T^3) \quad (862)$$

$$\tau^3_{\gamma,\alpha} = \sum_{a \in V} W^4_{a,\alpha} Y^1_{a,\gamma} \quad (2r_T r_V N_v) \quad (863)$$

$$\tau^4_{\gamma,\alpha} = \sum_{i \in O} W^3_{i,\alpha} Y^2_{i,\gamma} \quad (2r_T r_V N_o) \quad (864)$$

$$\tau^5_{\gamma,\alpha} = \sum_{\beta \in B} X_{\alpha,\beta} \tau^3_{\gamma,\beta} \tau^4_{\gamma,\beta} \quad (3r_T r_V^2) \quad (865)$$

$$\tau^6_{\gamma,\alpha} = \sum_{\delta \in A} Z_{\delta,\gamma} \tau^5_{\delta,\alpha} \quad (2r_T^2 r_V) \quad (866)$$

$$\tau^7_{\gamma,\alpha,w} = \sum_{\delta \in A} \tau^6_{\delta,\alpha} \tau^2_{\delta,\gamma,w} \quad (2r_D r_T^2 r_V) \quad (867)$$

$$\tau^8_{\alpha,i} = \sum_{a \in V} {}^1T_{a,i} W^2_{a,\alpha} \quad (2r_V N_o N_v) \quad (868)$$

$$\tau^9_{\gamma,\alpha,w} = \sum_{i \in O} {}^2D^2_{i,w} Y^{2,*}_{i,\gamma} \tau^8_{\alpha,i} \quad (3r_D r_T r_V N_o) \quad (869)$$

$$\tau^{10}_{\gamma,w,a} = \sum_{\alpha \in B} W^1_{a,\alpha} \tau^7_{\gamma,\alpha,w} \tau^9_{\gamma,\alpha,w} \quad (3r_D r_T r_V N_v) \quad (870)$$

$${}^{21}R_{a,\gamma} \leftarrow \sum_{w \in D} {}^2D^1_{a,w} \tau^{10}_{\gamma,w,a} \quad (2r_D r_T N_v) \quad (871)$$

Raw expression

$${}^{21}R_{a,\epsilon} \leftarrow - \sum_{\gamma \in A} \sum_{i \in O} \sum_{j \in O} \sum_{k \in O} \sum_{b \in V} \sum_{c \in V} \frac{1}{2} {}^1T_{b,k} Y^{2,*}_{i,\epsilon} Z^*_{\epsilon,\gamma} Y^{3,*}_{b,\gamma} Y^{4,*}_{j,\gamma} f_{k,c} {}^2D^{a,i,b,j} {}^2T_{a,i,c,j} \quad (872)$$

Factorized expression

$$\tau^0_{\gamma,\delta,w} = \sum_{i \in O} {}^2D^2_{i,w} Y^2_{i,\gamma} Y^{2,*}_{i,\delta} \quad (3r_D r_T^2 N_o) \quad (873)$$

$$\tau^1_{\alpha,i} = \sum_{a \in V} {}^1T_{a,i} W^2_{a,\alpha} \quad (2r_V N_o N_v) \quad (874)$$

$$\tau^2_{\gamma,\alpha,w} = \sum_{i \in O} {}^2D^4_{i,w} Y^{4,*}_{i,\gamma} \tau^1_{\alpha,i} \quad (3r_D r_T r_V N_o) \quad (875)$$

$$\tau^3_{\gamma,\alpha,w} = \sum_{a \in V} {}^2D^3_{a,w} W^1_{a,\alpha} Y^{3,*}_{a,\gamma} \quad (3r_D r_T r_V N_v) \quad (876)$$

$$\tau^4_{\gamma,\alpha} = \sum_{a \in V} W^4_{a,\alpha} Y^3_{a,\gamma} \quad (2r_T r_V N_v) \quad (877)$$

$$\tau^5_{\gamma,\alpha} = \sum_{i \in O} W^3_{i,\alpha} Y^4_{i,\gamma} \quad (2r_T r_V N_o) \quad (878)$$

$$\tau^6_{\gamma,\alpha} = \sum_{\beta \in B} X_{\alpha,\beta} \tau^4_{\gamma,\beta} \tau^5_{\gamma,\beta} \quad (3r_T r_V^2) \quad (879)$$

$$\tau^7_{\gamma,\alpha} = \sum_{\delta \in A} Z_{\gamma,\delta} \tau^6_{\delta,\alpha} \quad (2r_T^2 r_V) \quad (880)$$

$$\tau^8_{\gamma,\delta,w} = \sum_{\alpha \in B} \tau^7_{\gamma,\alpha} \tau^2_{\delta,\alpha,w} \tau^3_{\delta,\alpha,w} \quad (3r_D r_T^2 r_V) \quad (881)$$

$$\tau^9_{\gamma,\delta,w} = \sum_{\epsilon \in A} Z^*_{\delta,\epsilon} \tau^8_{\gamma,\epsilon,w} \quad (2r_D r_T^3) \quad (882)$$

$${}^{21}R_{a,\gamma} \leftarrow \sum_{\delta \in A} \sum_{w \in D} {}^2D^1_{a,w} Y^1_{a,\delta} \tau^0_{\delta,\gamma,w} \tau^9_{\delta,\gamma,w} \quad (4r_D r_T^2 N_v) \quad (883)$$

Raw expression

$${}^{21}R_{a,\epsilon} \leftarrow - \sum_{\gamma \in A} \sum_{i \in O} \sum_{j \in O} \sum_{k \in O} \sum_{b \in V} \sum_{c \in V} \frac{1}{2} {}^1T_{b,k} Y^{2,*}_{i,\epsilon} Z^*_{\epsilon,\gamma} Y^{3,*}_{b,\gamma} Y^{4,*}_{j,\gamma} f_{k,c} {}^2D^{a,i,b,j} {}^2T_{c,j,a,i} \quad (884)$$

Factorized expression

$$\tau^0_{\gamma,\delta,w} = \sum_{i \in O} {}^2D^2_{i,w} Y^4_{i,\gamma} Y^{2,*}_{i,\delta} \quad (3r_D r_T^2 N_o) \quad (885)$$

$$\tau^1_{\alpha,i} = \sum_{a \in V} {}^1T_{a,i} W^2_{a,\alpha} \quad (2r_V N_o N_v) \quad (886)$$

$$\tau^2_{\gamma,\alpha,w} = \sum_{i \in O} {}^2D^4_{i,w} Y^{4,*}_{i,\gamma} \tau^1_{\alpha,i} \quad (3r_D r_T r_V N_o) \quad (887)$$

$$\tau^3_{\gamma,\alpha,w} = \sum_{a \in V} {}^2D^3_{a,w} W^1_{a,\alpha} Y^{3,*}_{a,\gamma} \quad (3r_D r_T r_V N_v) \quad (888)$$

$$\tau^4_{\gamma,\alpha} = \sum_{a \in V} W^4_{a,\alpha} Y^1_{a,\gamma} \quad (2r_T r_V N_v) \quad (889)$$

$$\tau^5_{\gamma,\alpha} = \sum_{i \in O} W^3_{i,\alpha} Y^2_{i,\gamma} \quad (2r_T r_V N_o) \quad (890)$$

$$\tau^6_{\gamma,\alpha} = \sum_{\beta \in B} X_{\alpha,\beta} \tau^4_{\gamma,\beta} \tau^5_{\gamma,\beta} \quad (3r_T r_V^2) \quad (891)$$

$$\tau^7_{\gamma,\alpha} = \sum_{\delta \in A} Z_{\delta,\gamma} \tau^6_{\delta,\alpha} \quad (2r_T^2 r_V) \quad (892)$$

$$\tau^8_{\gamma,\delta,w} = \sum_{\epsilon \in A} Z_{\epsilon,\gamma} \tau^7_{\epsilon,\delta,w} \quad (2r_D r_T^3) \quad (905)$$

$$\tau^8_{\gamma,\delta,w} = \sum_{\alpha \in B} \tau^7_{\gamma,\alpha} \tau^2_{\delta,\alpha,w} \tau^3_{\delta,\alpha,w} \quad (3r_D r_T^2 r_V) \quad (893)$$

$$\tau^9_{\gamma,\delta,w} = \sum_{i \in O} {}^2D^2_{i,w} Y^4_{i,\gamma} Y^{2,*}_{i,\delta} \quad (3r_D r_T^2 N_o) \quad (906)$$

$$\tau^9_{\gamma,\delta,w} = \sum_{\epsilon \in A} Z^*_{\delta,\epsilon} \tau^8_{\gamma,\epsilon,w} \quad (2r_D r_T^3) \quad (894)$$

$${}^{21}R_{a,\gamma} \leftarrow \sum_{\delta \in A} \sum_{w \in D} {}^2D^1_{a,w} \tau^4_{\delta,a} \tau^8_{\delta,\gamma,w} \tau^9_{\delta,\gamma,w} \quad (4r_D r_T^2 N_v) \quad (907)$$

$${}^{21}R_{a,\gamma} \leftarrow \sum_{\delta \in A} \sum_{w \in D} {}^2D^1_{a,w} Y^3_{a,\delta} \tau^0_{\delta,\gamma,w} \tau^9_{\delta,\gamma,w} \quad (4r_D r_T^2 N_v) \quad \text{Raw expression} \quad (895)$$

$${}^{21}R_{a,\epsilon} \leftarrow - \sum_{\gamma \in A} \sum_{i \in O} \sum_{j \in O} \sum_{k \in O} \sum_{b \in V} \sum_{c \in V} \frac{1}{2} {}^1T_{c,i} Y^{2,*}_{i,\epsilon} Z^*_{\epsilon,\gamma} Y^{3,*}_{b,\gamma} Y^{4,*}_{j,\gamma} f_{k,c} {}^2D^{a,i,b,j} {}^2T_{b,j,a,k} \quad (908)$$

Raw expression

$${}^{21}R_{a,\epsilon} \leftarrow - \sum_{\gamma \in A} \sum_{i \in O} \sum_{j \in O} \sum_{k \in O} \sum_{b \in V} \sum_{c \in V} \frac{1}{2} {}^1T_{c,i} Y^{2,*}_{i,\epsilon} Z^*_{\epsilon,\gamma} Y^{3,*}_{b,\gamma} Y^{4,*}_{j,\gamma} f_{k,c} {}^2D^{a,i,b,j} {}^2T_{a,k,b,j} \quad (896)$$

Factorized expression

$$\tau^0_{\alpha,i} = \sum_{a \in V} {}^1T_{a,i} W^4_{a,\alpha} \quad (2r_V N_o N_v) \quad (909)$$

Factorized expression

$$\tau^0_{\alpha,i} = \sum_{a \in V} {}^1T_{a,i} W^4_{a,\alpha} \quad (2r_V N_o N_v) \quad (897)$$

$$\tau^1_{\alpha} = \sum_{i \in O} W^3_{i,\alpha} \tau^0_{\alpha,i} \quad (2r_V N_o) \quad (910)$$

$$\tau^1_{\alpha} = \sum_{i \in O} W^3_{i,\alpha} \tau^0_{\alpha,i} \quad (2r_V N_o) \quad (898)$$

$$\tau^2_{\alpha} = \sum_{\beta \in B} \tau^1_{\beta} X_{\alpha,\beta} \quad (2r_V^2) \quad (911)$$

$$\tau^2_{\alpha} = \sum_{\beta \in B} \tau^1_{\beta} X_{\alpha,\beta} \quad (2r_V^2) \quad (899)$$

$$\tau^3_{a,b} = \sum_{\alpha \in B} \tau^2_{\alpha} W^1_{a,\alpha} W^2_{b,\alpha} \quad (3r_V N_v^2) \quad (912)$$

$$\tau^3_{a,b} = \sum_{\alpha \in B} \tau^2_{\alpha} W^1_{a,\alpha} W^2_{b,\alpha} \quad (3r_V N_v^2) \quad (900)$$

$$\tau^4_{\gamma,a} = \sum_{b \in V} Y^1_{b,\gamma} \tau^3_{a,b} \quad (2r_T N_v^2) \quad (913)$$

$$\tau^4_{\gamma,a} = \sum_{b \in V} Y^3_{b,\gamma} \tau^3_{a,b} \quad (2r_T N_v^2) \quad (901)$$

$$\tau^5_{\gamma,\delta,w} = \sum_{i \in O} {}^2D^2_{i,w} Y^2_{i,\gamma} Y^{2,*}_{i,\delta} \quad (3r_D r_T^2 N_o) \quad (914)$$

$$\tau^5_{\gamma,\delta,w} = \sum_{a \in V} {}^2D^3_{a,w} Y^1_{a,\gamma} Y^{3,*}_{a,\delta} \quad (3r_D r_T^2 N_v) \quad (902)$$

$$\tau^6_{\gamma,\delta,w} = \sum_{a \in V} {}^2D^3_{a,w} Y^3_{a,\gamma} Y^{3,*}_{a,\delta} \quad (3r_D r_T^2 N_v) \quad (915)$$

$$\tau^6_{\gamma,\delta,w} = \sum_{i \in O} {}^2D^4_{i,w} Y^2_{i,\gamma} Y^{4,*}_{i,\delta} \quad (3r_D r_T^2 N_o) \quad (903)$$

$$\tau^7_{\gamma,\delta,w} = \sum_{i \in O} {}^2D^4_{i,w} Y^4_{i,\gamma} Y^{4,*}_{i,\delta} \quad (3r_D r_T^2 N_o) \quad (916)$$

$$\tau^7_{\gamma,\delta,w} = \sum_{\epsilon \in A} Z^*_{\delta,\epsilon} \tau^5_{\gamma,\epsilon,w} \tau^6_{\gamma,\epsilon,w} \quad (3r_D r_T^3) \quad (904)$$

$$\tau^8_{\gamma,\delta,w} = \sum_{\epsilon \in A} Z^*_{\delta,\epsilon} \tau^6_{\gamma,\epsilon,w} \tau^7_{\gamma,\epsilon,w} \quad (3r_D r_T^3) \quad (917)$$

$$\tau_{\gamma,\delta,w}^9 = \sum_{\epsilon \in A} Z_{\gamma,\epsilon} \tau_{\epsilon,\delta,w}^8 \quad (2r_D r_T^3) \quad (918)$$

$${}^{21}R_{a,\gamma} \leftarrow \sum_{\delta \in A} \sum_{w \in D} {}^2D_{a,w}^1 \tau_{\delta,a}^4 \tau_{\delta,\gamma,w}^5 \tau_{\delta,\gamma,w}^9 \quad (4r_D r_T^2 N_v) \quad (919)$$

Raw expression

$${}^{21}R_{a,\epsilon} \leftarrow - \sum_{\gamma \in A} \sum_{i \in O} \sum_{j \in O} \sum_{k \in O} \sum_{b \in V} \sum_{c \in V} \frac{1}{2} {}^1T_{c,j} Y^{2,*}_{i,\epsilon} Z^*_{\epsilon,\gamma} Y^{3,*}_{b,\gamma} Y^{4,*}_{j,\gamma} f_{k,c} {}^2D^{a,i,b,j} {}^2T_{a,i,b,k} \quad (920)$$

Factorized expression

$$\tau_{\gamma,\delta,w}^0 = \sum_{i \in O} {}^2D^2_{i,w} Y^2_{i,\gamma} Y^{2,*}_{i,\delta} \quad (3r_D r_T^2 N_o) \quad (921)$$

$$\tau_{\gamma,\delta,w}^1 = \sum_{i \in O} {}^2D^4_{i,w} Y^4_{i,\gamma} Y^{4,*}_{i,\delta} \quad (3r_D r_T^2 N_o) \quad (922)$$

$$\tau_{\alpha,i}^2 = \sum_{a \in V} {}^1T_{a,i} W^4_{a,\alpha} \quad (2r_V N_o N_v) \quad (923)$$

$$\tau_{\alpha}^3 = \sum_{i \in O} W^3_{i,\alpha} \tau_{\alpha,i}^2 \quad (2r_V N_o) \quad (924)$$

$$\tau_{\alpha}^4 = \sum_{\beta \in B} \tau_{\beta}^3 X_{\alpha,\beta} \quad (2r_V^2) \quad (925)$$

$$\tau_{a,b}^5 = \sum_{\alpha \in B} \tau_{\alpha}^4 W^1_{a,\alpha} W^2_{b,\alpha} \quad (3r_V N_v^2) \quad (926)$$

$$\tau_{\gamma,a}^6 = \sum_{b \in V} Y^3_{b,\gamma} \tau_{a,b}^5 \quad (2r_T N_v^2) \quad (927)$$

$$\tau_{\gamma,\delta,w}^7 = \sum_{a \in V} {}^2D^3_{a,w} Y^{3,*}_{a,\delta} \tau_{\gamma,a}^6 \quad (3r_D r_T^2 N_v) \quad (928)$$

$$\tau_{\gamma,\delta,w}^8 = \sum_{\epsilon \in A} Z^*_{\delta,\epsilon} \tau_{\gamma,\epsilon,w}^1 \tau_{\gamma,\epsilon,w}^7 \quad (3r_D r_T^3) \quad (929)$$

$$\tau_{\gamma,\delta,w}^9 = \sum_{\epsilon \in A} Z_{\gamma,\epsilon} \tau_{\epsilon,\delta,w}^8 \quad (2r_D r_T^3) \quad (930)$$

$${}^{21}R_{a,\gamma} \leftarrow \sum_{\delta \in A} \sum_{w \in D} {}^2D^1_{a,w} Y^1_{a,\delta} \tau_{\delta,\gamma,w}^0 \tau_{\delta,\gamma,w}^9 \quad (4r_D r_T^2 N_v) \quad (931)$$

Raw expression

$${}^{21}R_{a,\epsilon} \leftarrow - \sum_{\gamma \in A} \sum_{i \in O} \sum_{j \in O} \sum_{k \in O} \sum_{b \in V} \sum_{c \in V} \frac{1}{2} {}^1T_{c,j} Y^{2,*}_{i,\epsilon} Z^*_{\epsilon,\gamma} Y^{3,*}_{b,\gamma} Y^{4,*}_{j,\gamma} f_{k,c} {}^2D^{a,i,b,j} {}^2T_{b,k,a,i} \quad (932)$$

Factorized expression

$$\tau_{\gamma,\delta,w}^0 = \sum_{i \in O} {}^2D^4_{i,w} Y^2_{i,\gamma} Y^{4,*}_{i,\delta} \quad (3r_D r_T^2 N_o) \quad (933)$$

$$\tau_{\alpha,i}^1 = \sum_{a \in V} {}^1T_{a,i} W^4_{a,\alpha} \quad (2r_V N_o N_v) \quad (934)$$

$$\tau_{\alpha}^2 = \sum_{i \in O} W^3_{i,\alpha} \tau_{\alpha,i}^1 \quad (2r_V N_o) \quad (935)$$

$$\tau_{\alpha}^3 = \sum_{\beta \in B} \tau_{\beta}^2 X_{\alpha,\beta} \quad (2r_V^2) \quad (936)$$

$$\tau_{a,b}^4 = \sum_{\alpha \in B} \tau_{\alpha}^3 W^1_{a,\alpha} W^2_{b,\alpha} \quad (3r_V N_v^2) \quad (937)$$

$$\tau_{\gamma,a}^5 = \sum_{b \in V} Y^1_{b,\gamma} \tau_{a,b}^4 \quad (2r_T N_v^2) \quad (938)$$

$$\tau_{\gamma,\delta,w}^6 = \sum_{a \in V} {}^2D^3_{a,w} Y^{3,*}_{a,\delta} \tau_{\gamma,a}^5 \quad (3r_D r_T^2 N_v) \quad (939)$$

$$\tau_{\gamma,\delta,w}^7 = \sum_{\epsilon \in A} Z^*_{\delta,\epsilon} \tau_{\gamma,\epsilon,w}^0 \tau_{\gamma,\epsilon,w}^6 \quad (3r_D r_T^3) \quad (940)$$

$$\tau_{\gamma,\delta,w}^8 = \sum_{\epsilon \in A} Z_{\epsilon,\gamma} \tau_{\epsilon,\delta,w}^7 \quad (2r_D r_T^3) \quad (941)$$

$$\tau_{\gamma,\delta,w}^9 = \sum_{i \in O} {}^2D^2_{i,w} Y^4_{i,\gamma} Y^{2,*}_{i,\delta} \quad (3r_D r_T^2 N_o) \quad (942)$$

$${}^{21}R_{a,\gamma} \leftarrow \sum_{\delta \in A} \sum_{w \in D} {}^2D^1_{a,w} Y^3_{a,\delta} \tau_{\delta,\gamma,w}^8 \tau_{\delta,\gamma,w}^9 \quad (4r_D r_T^2 N_v) \quad (943)$$

Raw expression

$${}^{21}R_{a,\epsilon} \leftarrow \sum_{\gamma \in A} \sum_{i \in O} \sum_{j \in O} \sum_{k \in O} \sum_{l \in O} \sum_{b \in V} \sum_{c \in V} \frac{1}{2} {}^1T_{a,k} Y^{2,*}_{i,\epsilon} Z^*_{\epsilon,\gamma} Y^{3,*}_{b,\gamma} Y^{4,*}_{j,\gamma} {}^2D^{a,i,b,j} {}^2T_{b,j,c,l} V_{l,i,k,c} \quad (944)$$

Factorized expression

$$\tau^0_{\gamma,\alpha,w} = \sum_{a \in V} {}^2D^3_{a,w} W^1_{a,\alpha} Y^{3,*}_{a,\gamma} \quad (3r_D r_T r_V N_v) \quad (945)$$

$$\tau^1_{\gamma,\alpha} = \sum_{a \in V} W^2_{a,\alpha} Y^1_{a,\gamma} \quad (2r_T r_V N_v) \quad (946)$$

$$\tau^2_{\gamma,\alpha,i} = \sum_{\delta \in A} Y^2_{i,\delta} Z_{\delta,\gamma} \tau^1_{\delta,\alpha} \quad (3r_T^2 r_V N_o) \quad (947)$$

$$\tau^3_{\gamma,\delta,\alpha,w} = \sum_{i \in O} {}^2D^4_{i,w} Y^{4,*}_{i,\delta} \tau^0_{\delta,\alpha,w} \tau^2_{\gamma,\alpha,i} \quad (4r_D r_T^2 r_V N_o) \quad (948)$$

$$\tau^4_{\gamma,\alpha} = \sum_{a \in V} W^4_{a,\alpha} Y^3_{a,\gamma} \quad (2r_T r_V N_v) \quad (949)$$

$$\tau^5_{\gamma,\alpha,i} = \sum_{\beta \in B} X_{\alpha,\beta} W^3_{i,\beta} \tau^4_{\gamma,\beta} \quad (3r_T r_V^2 N_o) \quad (950)$$

$$\tau^6_{\gamma,\delta,w,i} = \sum_{\alpha \in B} \tau^5_{\gamma,\alpha,i} \tau^3_{\gamma,\delta,\alpha,w} \quad (2r_D r_T^2 r_V N_o) \quad (951)$$

$$\tau^7_{\gamma,w,i,j} = \sum_{\delta \in A} {}^2D^2_{i,w} Y^4_{i,\delta} \tau^6_{\delta,\gamma,w,j} \quad (3r_D r_T^2 N_o^2) \quad (952)$$

$$\tau^8_{\gamma,w,i} = \sum_{\delta \in A} \sum_{j \in O} Y^{2,*}_{j,\gamma} Z^*_{\gamma,\delta} \tau^7_{\delta,w,j,i} \quad (3r_D r_T^2 N_o^2) \quad (953)$$

$${}^{21}R_{a,\gamma} \leftarrow - \sum_{w \in D} \sum_{i \in O} \frac{1}{2} D^1_{a,w} {}^1T_{a,i} \tau^8_{\gamma,w,i} \quad (3r_D r_T N_o N_v) \quad (954)$$

Raw expression

$${}^{21}R_{a,\epsilon} \leftarrow \sum_{\gamma \in A} \sum_{i \in O} \sum_{j \in O} \sum_{k \in O} \sum_{l \in O} \sum_{b \in V} \sum_{c \in V} \frac{1}{2} {}^1T_{a,k} Y^{2,*}_{i,\epsilon} Z^*_{\epsilon,\gamma} Y^{3,*}_{b,\gamma} Y^{4,*}_{j,\gamma} {}^2D^{a,i,b,j} {}^2T_{b,l,c,i} V_{k,i,l,j} \quad (955)$$

Factorized expression

$$\tau^0_{\gamma,\alpha,w} = \sum_{a \in V} {}^2D^3_{a,w} W^1_{a,\alpha} Y^{3,*}_{a,\gamma} \quad (3r_D r_T r_V N_v) \quad (956)$$

$$\tau^1_{\gamma,\alpha} = \sum_{a \in V} W^2_{a,\alpha} Y^3_{a,\gamma} \quad (2r_T r_V N_v) \quad (957)$$

$$\tau^2_{\gamma,\alpha,i} = \sum_{\delta \in A} Z_{\gamma,\delta} Y^4_{i,\delta} \tau^1_{\delta,\alpha} \quad (3r_T^2 r_V N_o) \quad (958)$$

$$\tau^3_{\gamma,\delta,\alpha,w} = \sum_{i \in O} {}^2D^4_{i,w} Y^{4,*}_{i,\delta} \tau^0_{\delta,\alpha,w} \tau^2_{\gamma,\alpha,i} \quad (4r_D r_T^2 r_V N_o) \quad (959)$$

$$\tau^4_{\gamma,\alpha} = \sum_{a \in V} W^4_{a,\alpha} Y^1_{a,\gamma} \quad (2r_T r_V N_v) \quad (960)$$

$$\tau^5_{\gamma,\alpha,i} = \sum_{\beta \in B} X_{\alpha,\beta} W^3_{i,\beta} \tau^4_{\gamma,\beta} \quad (3r_T r_V^2 N_o) \quad (961)$$

$$\tau^6_{\gamma,\delta,w,i} = \sum_{\alpha \in B} \tau^5_{\gamma,\alpha,i} \tau^3_{\gamma,\delta,\alpha,w} \quad (2r_D r_T^2 r_V N_o) \quad (962)$$

$$\tau^7_{\gamma,w,i,j} = \sum_{\delta \in A} {}^2D^2_{i,w} Y^2_{i,\delta} \tau^6_{\delta,\gamma,w,j} \quad (3r_D r_T^2 N_o^2) \quad (963)$$

$$\tau^8_{\gamma,w,i} = \sum_{\delta \in A} \sum_{j \in O} Y^{2,*}_{j,\gamma} Z^*_{\gamma,\delta} \tau^7_{\delta,w,j,i} \quad (3r_D r_T^2 N_o^2) \quad (964)$$

$${}^{21}R_{a,\gamma} \leftarrow - \sum_{w \in D} \sum_{i \in O} \frac{1}{2} D^1_{a,w} {}^1T_{a,i} \tau^8_{\gamma,w,i} \quad (3r_D r_T N_o N_v) \quad (965)$$

Raw expression

$${}^{21}R_{a,\epsilon} \leftarrow \sum_{\gamma \in A} \sum_{i \in O} \sum_{j \in O} \sum_{k \in O} \sum_{l \in O} \sum_{b \in V} \sum_{c \in V} \frac{1}{2} {}^1T_{a,k} Y^{2,*}_{i,\epsilon} Z^*_{\epsilon,\gamma} Y^{3,*}_{b,\gamma} Y^{4,*}_{j,\gamma} {}^2D^{a,i,b,j} {}^2T_{b,l,c,j} V_{k,i,l,c} \quad (966)$$

Factorized expression

$$\tau^0_{\gamma,\alpha} = \sum_{a \in V} W^2_{a,\alpha} Y^1_{a,\gamma} \quad (2r_T r_V N_v) \quad (967)$$

$$\tau^1_{\gamma,\alpha,i} = \sum_{\delta \in A} Y^2_{i,\delta} Z_{\delta,\gamma} \tau^0_{\delta,\alpha} \quad (3r_T^2 r_V N_o) \quad (968)$$

$$\tau^1_{\gamma,\alpha,i} = \sum_{\delta \in A} Z_{\gamma,\delta} Y^4_{i,\delta} \tau^0_{\delta,\alpha} \quad (3r_T^2 r_V N_o) \quad (981)$$

$$\tau^2_{\gamma,w,i} = \sum_{a \in V} {}^2D^3_{a,w} {}^1T_{a,i} Y^{3,*}_{a,\gamma} \quad (3r_D r_T N_o N_v) \quad (969)$$

$$\tau^2_{\gamma,w,i} = \sum_{a \in V} {}^2D^3_{a,w} {}^1T_{a,i} Y^{3,*}_{a,\gamma} \quad (3r_D r_T N_o N_v) \quad (982)$$

$$\tau^3_{\gamma,w,i,j} = \sum_{\delta \in A} Z^*_{\gamma,\delta} Y^{4,*}_{j,\delta} \tau^2_{\delta,w,i} \quad (3r_D r_T^2 N_o^2) \quad (970)$$

$$\tau^3_{\gamma,w,i,j} = \sum_{\delta \in A} Z^*_{\gamma,\delta} Y^{4,*}_{j,\delta} \tau^2_{\delta,w,i} \quad (3r_D r_T^2 N_o^2) \quad (983)$$

$$\tau^4_{\gamma,\delta,w,i} = \sum_{j \in O} {}^2D^4_{j,w} Y^4_{j,\gamma} \tau^3_{\delta,w,i,j} \quad (3r_D r_T^2 N_o^2) \quad (971)$$

$$\tau^4_{\gamma,\delta,w,i} = \sum_{j \in O} {}^2D^4_{j,w} Y^2_{j,\gamma} \tau^3_{\delta,w,i,j} \quad (3r_D r_T^2 N_o^2) \quad (984)$$

$$\tau^5_{\gamma,\alpha} = \sum_{a \in V} W^4_{a,\alpha} Y^3_{a,\gamma} \quad (2r_T r_V N_v) \quad (972)$$

$$\tau^5_{\gamma,\alpha} = \sum_{a \in V} W^4_{a,\alpha} Y^1_{a,\gamma} \quad (2r_T r_V N_v) \quad (985)$$

$$\tau^6_{\gamma,\alpha,i} = \sum_{\beta \in B} X_{\alpha,\beta} W^3_{i,\beta} \tau^5_{\gamma,\beta} \quad (3r_T r_V^2 N_o) \quad (973)$$

$$\tau^6_{\gamma,\alpha,i} = \sum_{\beta \in B} X_{\alpha,\beta} W^3_{i,\beta} \tau^5_{\gamma,\beta} \quad (3r_T r_V^2 N_o) \quad (986)$$

$$\tau^7_{\gamma,\delta,\alpha,w} = \sum_{i \in O} \tau^6_{\gamma,\alpha,i} \tau^4_{\gamma,\delta,w,i} \quad (2r_D r_T^2 r_V N_o) \quad (974)$$

$$\tau^7_{\gamma,\delta,\alpha,w} = \sum_{i \in O} \tau^6_{\gamma,\alpha,i} \tau^4_{\gamma,\delta,w,i} \quad (2r_D r_T^2 r_V N_o) \quad (987)$$

$$\tau^8_{\gamma,\alpha,w,i} = \sum_{\delta \in A} \tau^1_{\delta,\alpha,i} \tau^7_{\delta,\gamma,\alpha,w} \quad (2r_D r_T^2 r_V N_o) \quad (975)$$

$$\tau^8_{\gamma,\alpha,w,i} = \sum_{\delta \in A} \tau^1_{\delta,\alpha,i} \tau^7_{\delta,\gamma,\alpha,w} \quad (2r_D r_T^2 r_V N_o) \quad (988)$$

$$\tau^9_{\gamma,\alpha,w} = \sum_{i \in O} {}^2D^2_{i,w} Y^{2,*}_{i,\gamma} \tau^8_{\gamma,\alpha,w,i} \quad (3r_D r_T r_V N_o) \quad (976)$$

$$\tau^9_{\gamma,\alpha,w} = \sum_{i \in O} {}^2D^2_{i,w} Y^{2,*}_{i,\gamma} \tau^8_{\gamma,\alpha,w,i} \quad (3r_D r_T r_V N_o) \quad (989)$$

$$\tau^{10}_{\gamma,w,a} = \sum_{\alpha \in B} W^1_{a,\alpha} \tau^9_{\gamma,\alpha,w} \quad (2r_D r_T r_V N_v) \quad (977)$$

$$\tau^{10}_{\gamma,w,a} = \sum_{\alpha \in B} W^1_{a,\alpha} \tau^9_{\gamma,\alpha,w} \quad (2r_D r_T r_V N_v) \quad (990)$$

$${}^{21}R_{a,\gamma} \leftarrow - \sum_{w \in D} \frac{1}{2} {}^2D^1_{a,w} \tau^{10}_{\gamma,w,a} \quad (2r_D r_T N_v) \quad (978)$$

$${}^{21}R_{a,\gamma} \leftarrow - \sum_{w \in D} \frac{1}{2} {}^2D^1_{a,w} \tau^{10}_{\gamma,w,a} \quad (2r_D r_T N_v) \quad (991)$$

Raw expression

$${}^{21}R_{a,\epsilon} \leftarrow \sum_{\gamma \in A} \sum_{i \in O} \sum_{j \in O} \sum_{k \in O} \sum_{l \in O} \sum_{b \in V} \sum_{c \in V} \frac{1}{2} {}^1T_{a,k} Y^{2,*}_{i,\epsilon} Z^*_{\epsilon,\gamma} Y^{3,*}_{b,\gamma} Y^{4,*}_{j,\gamma} {}^2D^{a,i,b,j} {}^2T_{c,i,b,l} V_{k,c,l,j} \quad (979)$$

Raw expression

$${}^{21}R_{a,\epsilon} \leftarrow \sum_{\gamma \in A} \sum_{i \in O} \sum_{j \in O} \sum_{k \in O} \sum_{l \in O} \sum_{b \in V} \sum_{c \in V} \frac{1}{2} {}^1T_{a,k} Y^{2,*}_{i,\epsilon} Z^*_{\epsilon,\gamma} Y^{3,*}_{b,\gamma} Y^{4,*}_{j,\gamma} {}^2D^{a,i,b,j} {}^2T_{c,j,b,l} V_{k,i,l,c} \quad (992)$$

Factorized expression

$$\tau^0_{\gamma,\alpha} = \sum_{a \in V} W^2_{a,\alpha} Y^3_{a,\gamma} \quad (2r_T r_V N_v) \quad (980)$$

Factorized expression

$$\tau^0_{\gamma,\delta,w} = \sum_{a \in V} {}^2D^3_{a,w} Y^1_{a,\gamma} Y^{3,*}_{a,\delta} \quad (3r_D r_T^2 N_v) \quad (993)$$



$$\tau^1_{\gamma,\alpha} = \sum_{i \in O} W^3_{i,\alpha} Y^2_{i,\gamma} \quad (2r_T r_V N_o) \quad (994)$$

$$\tau^2_{\gamma,\alpha,i} = \sum_{\delta \in A} Y^2_{i,\delta} Z_{\delta,\gamma} \tau^1_{\delta,\alpha} \quad (3r_T^2 r_V N_o) \quad (1007)$$

$$\tau^2_{\gamma,\alpha} = \sum_{a \in V} W^4_{a,\alpha} Y^3_{a,\gamma} \quad (2r_T r_V N_v) \quad (995)$$

$$\tau^3_{\gamma,\alpha} = \sum_{i \in O} W^3_{i,\alpha} Y^4_{i,\gamma} \quad (2r_T r_V N_o) \quad (1008)$$

$$\tau^3_{\gamma,\alpha,i} = \sum_{\delta \in A} Z_{\gamma,\delta} Y^4_{i,\delta} \tau^2_{\delta,\alpha} \quad (3r_T^2 r_V N_o) \quad (996)$$

$$\tau^4_{\gamma,\alpha,w} = \sum_{\delta \in A} \sum_{i \in O} {}^2D^4_{i,w} Y^{4,*}_{i,\gamma} \tau^3_{\delta,\alpha} \tau^0_{\delta,\gamma,w} \tau^2_{\delta,\alpha,i} \quad (5r_D r_T^2 r_V N_o) \quad (1009)$$

$$\tau^4_{\gamma,\alpha,w} = \sum_{\delta \in A} \sum_{i \in O} {}^2D^4_{i,w} Y^{4,*}_{i,\gamma} \tau^1_{\delta,\alpha} \tau^0_{\delta,\gamma,w} \tau^3_{\delta,\alpha,i} \quad (5r_D r_T^2 r_V N_o) \quad (997)$$

$$\tau^5_{\gamma,\alpha,w} = \sum_{\beta \in B} X_{\alpha,\beta} \tau^4_{\gamma,\beta,w} \quad (2r_D r_T r_V^2) \quad (1010)$$

$$\tau^5_{\gamma,\alpha,w} = \sum_{\beta \in B} X_{\alpha,\beta} \tau^4_{\gamma,\beta,w} \quad (2r_D r_T r_V^2) \quad (998)$$

$$\tau^6_{\gamma,\alpha,w} = \sum_{\delta \in A} Z^*_{\gamma,\delta} \tau^5_{\delta,\alpha,w} \quad (2r_D r_T^2 r_V) \quad (1011)$$

$$\tau^6_{\gamma,\alpha,w} = \sum_{\delta \in A} Z^*_{\gamma,\delta} \tau^5_{\delta,\alpha,w} \quad (2r_D r_T^2 r_V) \quad (999)$$

$$\tau^7_{\alpha,i} = \sum_{a \in V} {}^1T_{a,i} W^2_{a,\alpha} \quad (2r_V N_o N_v) \quad (1012)$$

$$\tau^7_{\alpha,i} = \sum_{a \in V} {}^1T_{a,i} W^2_{a,\alpha} \quad (2r_V N_o N_v) \quad (1000)$$

$$\tau^8_{\gamma,\alpha,w} = \sum_{i \in O} {}^2D^2_{i,w} Y^{2,*}_{i,\gamma} \tau^7_{\alpha,i} \quad (3r_D r_T r_V N_o) \quad (1013)$$

$$\tau^8_{\gamma,\alpha,w} = \sum_{i \in O} {}^2D^2_{i,w} Y^{2,*}_{i,\gamma} \tau^7_{\alpha,i} \quad (3r_D r_T r_V N_o) \quad (1001)$$

$$\tau^9_{\gamma,w,a} = \sum_{\alpha \in B} W^1_{a,\alpha} \tau^6_{\gamma,\alpha,w} \tau^8_{\gamma,\alpha,w} \quad (3r_D r_T r_V N_v) \quad (1014)$$

$$\tau^9_{\gamma,w,a} = \sum_{\alpha \in B} W^1_{a,\alpha} \tau^6_{\gamma,\alpha,w} \tau^8_{\gamma,\alpha,w} \quad (3r_D r_T r_V N_v) \quad (1002)$$

$${}^{21}R_{a,\gamma} \leftarrow - \sum_{w \in D} \frac{1}{2} {}^2D^1_{a,w} \tau^9_{\gamma,w,a} \quad (2r_D r_T N_v) \quad (1015)$$

$${}^{21}R_{a,\gamma} \leftarrow - \sum_{w \in D} \frac{1}{2} {}^2D^1_{a,w} \tau^9_{\gamma,w,a} \quad (2r_D r_T N_v) \quad (1003)$$

Raw expression

$${}^{21}R_{a,\epsilon} \leftarrow \sum_{\gamma \in A} \sum_{i \in O} \sum_{j \in O} \sum_{k \in O} \sum_{l \in O} \sum_{b \in V} \sum_{c \in V} \frac{1}{2} {}^1T_{a,k} Y^{2,*}_{i,\epsilon} Z^*_{\epsilon,\gamma} Y^{3,*}_{b,\gamma} Y^{4,*}_{j,\gamma} {}^2D^{a,i,b,j} {}^2T_{c,l,b,j} V_{l,i,k,c} \quad (1004)$$

Factorized expression

$$\tau^0_{\gamma,\delta,w} = \sum_{a \in V} {}^2D^3_{a,w} Y^3_{a,\gamma} Y^{3,*}_{a,\delta} \quad (3r_D r_T^2 N_v) \quad (1005)$$

$$\tau^1_{\gamma,\alpha} = \sum_{a \in V} W^4_{a,\alpha} Y^1_{a,\gamma} \quad (2r_T r_V N_v) \quad (1006)$$

Raw expression

$${}^{21}R_{a,\epsilon} \leftarrow \sum_{\gamma \in A} \sum_{i \in O} \sum_{j \in O} \sum_{k \in O} \sum_{l \in O} \sum_{b \in V} \sum_{c \in V} \frac{1}{2} {}^1T_{b,k} Y^{2,*}_{i,\epsilon} Z^*_{\epsilon,\gamma} Y^{3,*}_{b,\gamma} Y^{4,*}_{j,\gamma} {}^2D^{a,i,b,j} {}^2T_{a,i,c,l} V_{k,c,l,j} \quad (1016)$$

Factorized expression

$$\tau^0_{\gamma,\delta,w} = \sum_{a \in V} {}^2D^3_{a,w} Y^1_{a,\gamma} Y^{3,*}_{a,\delta} \quad (3r_D r_T^2 N_v) \quad (1017)$$

$$\tau^1_{\gamma,\delta,w} = \sum_{i \in O} {}^2D^4_{i,w} Y^2_{i,\gamma} Y^{4,*}_{i,\delta} \quad (3r_D r_T^2 N_o) \quad (1018)$$

$$\tau^2_{\gamma,\delta,w} = \sum_{\epsilon \in A} Z^*_{\delta,\epsilon} \tau^0_{\gamma,\epsilon,w} \tau^1_{\gamma,\epsilon,w} \quad (3r_D r_T^3) \quad (1019)$$

$$\tau^3_{\gamma,\delta,w} = \sum_{\epsilon \in A} Z_{\epsilon,\gamma} \tau^2_{\epsilon,\delta,w} \quad (2r_D r_T^3) \quad (1020)$$

$$\tau^4_{\alpha,i} = \sum_{a \in V} {}^1T_{a,i} W^4_{a,\alpha} \quad (2r_V N_o N_v) \quad (1033)$$

$$\tau^4_{\alpha,i} = \sum_{a \in V} {}^1T_{a,i} W^4_{a,\alpha} \quad (2r_V N_o N_v) \quad (1021)$$

$$\tau^5_{\alpha,i,j} = \sum_{\beta \in B} X_{\alpha,\beta} W^3_{j,\beta} \tau^4_{\beta,i} \quad (3r_V^2 N_o^2) \quad (1034)$$

$$\tau^5_{\alpha,i,j} = \sum_{\beta \in B} X_{\alpha,\beta} W^3_{j,\beta} \tau^4_{\beta,i} \quad (3r_V^2 N_o^2) \quad (1022)$$

$$\tau^6_{\gamma,\alpha,i} = \sum_{j \in O} Y^2_{j,\gamma} \tau^5_{\alpha,i,j} \quad (2r_T r_V N_o^2) \quad (1035)$$

$$\tau^6_{\gamma,\alpha,i} = \sum_{j \in O} Y^4_{j,\gamma} \tau^5_{\alpha,i,j} \quad (2r_T r_V N_o^2) \quad (1023)$$

$$\tau^7_{\gamma,\alpha} = \sum_{a \in V} W^2_{a,\alpha} Y^1_{a,\gamma} \quad (2r_T r_V N_v) \quad (1036)$$

$$\tau^7_{\gamma,\alpha} = \sum_{a \in V} W^2_{a,\alpha} Y^3_{a,\gamma} \quad (2r_T r_V N_v) \quad (1024)$$

$$\tau^8_{\gamma,i,a} = \sum_{\alpha \in B} W^1_{a,\alpha} \tau^7_{\gamma,\alpha} \tau^6_{\gamma,\alpha,i} \quad (3r_T r_V N_o N_v) \quad (1037)$$

$$\tau^8_{\gamma,i,a} = \sum_{\alpha \in B} W^1_{a,\alpha} \tau^7_{\gamma,\alpha} \tau^6_{\gamma,\alpha,i} \quad (3r_T r_V N_o N_v) \quad (1025)$$

$$\tau^9_{\gamma,w,a} = \sum_{\delta \in A} \sum_{i \in O} {}^2D^2_{i,w} Y^{2,*}_{i,\gamma} \tau^3_{\delta,\gamma,w} \tau^8_{\delta,i,a} \quad (4r_D r_T^2 N_o N_v) \quad (1038)$$

$$\tau^9_{\gamma,w,a} = \sum_{\delta \in A} \sum_{i \in O} {}^2D^2_{i,w} Y^{2,*}_{i,\gamma} \tau^3_{\delta,\gamma,w} \tau^8_{\delta,i,a} \quad (4r_D r_T^2 N_o N_v) \quad {}^{21}R_{a,\gamma} \leftarrow - \sum_{w \in D} \frac{1}{2} {}^2D^1_{a,w} \tau^9_{\gamma,w,a} \quad (2r_D r_T N_v) \quad (1039)$$

Raw expression

$${}^{21}R_{a,\gamma} \leftarrow - \sum_{w \in D} \frac{1}{2} {}^2D^1_{a,w} \tau^9_{\gamma,w,a} \quad (2r_D r_T N_v) \quad (1027)$$

$${}^{21}R_{a,\epsilon} \leftarrow \sum_{\gamma \in A} \sum_{i \in O} \sum_{j \in O} \sum_{k \in O} \sum_{l \in O} \sum_{b \in V} \sum_{c \in V} \frac{1}{2} {}^1T_{b,k} Y^{2,*}_{i,\epsilon} Z^{*,\gamma}_{\epsilon,\gamma} Y^{3,*}_{b,\gamma} Y^{4,*}_{j,\gamma} {}^2D^{a,i,b,j} {}^2T_{a,l,c,j} V_{l,i,k,c} \quad (1040)$$

Raw expression

$${}^{21}R_{a,\epsilon} \leftarrow \sum_{\gamma \in A} \sum_{i \in O} \sum_{j \in O} \sum_{k \in O} \sum_{l \in O} \sum_{b \in V} \sum_{c \in V} \frac{1}{2} {}^1T_{b,k} Y^{2,*}_{i,\epsilon} Z^{*,\gamma}_{\epsilon,\gamma} Y^{3,*}_{b,\gamma} Y^{4,*}_{j,\gamma} {}^2D^{a,i,b,j} {}^2T_{a,l,c,j} V_{l,i,k,c} \quad (1028)$$

Factorized expression

$$\tau^0_{\gamma,\alpha,w} = \sum_{a \in V} {}^2D^3_{a,w} W^1_{a,\alpha} Y^{3,*}_{a,\gamma} \quad (3r_D r_T r_V N_v) \quad (1041)$$

Factorized expression

$$\tau^0_{\gamma,\delta,w} = \sum_{a \in V} {}^2D^3_{a,w} Y^3_{a,\gamma} Y^{3,*}_{a,\delta} \quad (3r_D r_T^2 N_v) \quad (1029)$$

$$\tau^1_{\gamma,\alpha} = \sum_{a \in V} W^2_{a,\alpha} Y^3_{a,\gamma} \quad (2r_T r_V N_v) \quad (1042)$$

$$\tau^1_{\gamma,\delta,w} = \sum_{i \in O} {}^2D^4_{i,w} Y^4_{i,\gamma} Y^{4,*}_{i,\delta} \quad (3r_D r_T^2 N_o) \quad (1030)$$

$$\tau^2_{\gamma,\alpha,i} = \sum_{\delta \in A} Z_{\gamma,\delta} Y^4_{i,\delta} \tau^1_{\delta,\alpha} \quad (3r_T^2 r_V N_o) \quad (1043)$$

$$\tau^2_{\gamma,\delta,w} = \sum_{\epsilon \in A} Z^*_{\delta,\epsilon} \tau^0_{\gamma,\epsilon,w} \tau^1_{\gamma,\epsilon,w} \quad (3r_D r_T^3) \quad (1031)$$

$$\tau^3_{\gamma,\delta,\alpha,w} = \sum_{i \in O} {}^2D^4_{i,w} Y^{4,*}_{i,\delta} \tau^0_{\delta,\alpha,w} \tau^2_{\gamma,\alpha,i} \quad (4r_D r_T^2 r_V N_o) \quad (1044)$$

$$\tau^3_{\gamma,\delta,w} = \sum_{\epsilon \in A} Z_{\gamma,\epsilon} \tau^2_{\epsilon,\delta,w} \quad (2r_D r_T^3) \quad (1032)$$

$$\tau^4_{\alpha,i} = \sum_{a \in V} {}^1T_{a,i} W^4_{a,\alpha} \quad (2r_V N_o N_v) \quad (1045)$$

$$\tau^5_{\alpha,i,j} = \sum_{\beta \in B} X_{\alpha,\beta} W^3_{j,\beta} \tau^4_{\beta,i} \quad (3r_V^2 N_o^2) \quad (1046)$$

$$\tau^6_{\gamma,\alpha,i} = \sum_{j \in O} Y^2_{j,\gamma} \tau^5_{\alpha,i,j} \quad (2r_T r_V N_o^2) \quad (1047)$$

$$\tau^7_{\gamma,\delta,w,i} = \sum_{\alpha \in B} \tau^6_{\gamma,\alpha,i} \tau^3_{\gamma,\delta,\alpha,w} \quad (2r_D r_T^2 r_V N_o) \quad (1048)$$

$$\tau^8_{\gamma,\delta,w} = \sum_{\epsilon \in A} \sum_{i \in O} {}^2D^2_{i,w} Y^{2,*}_{i,\delta} Z^*_{\delta,\epsilon} \tau^7_{\gamma,\epsilon,w,i} \quad (4r_D r_T^3 N_o) \quad (1049)$$

$${}^{21}R_{a,\gamma} \leftarrow - \sum_{\delta \in A} \sum_{w \in D} \frac{1}{2} D^1_{a,w} Y^1_{a,\delta} \tau^8_{\delta,\gamma,w} \quad (3r_D r_T^2 N_v) \quad (1050)$$

Raw expression

$${}^{21}R_{a,\epsilon} \leftarrow \sum_{\gamma \in A} \sum_{i \in O} \sum_{j \in O} \sum_{k \in O} \sum_{l \in O} \sum_{b \in V} \sum_{c \in V} \frac{1}{2} {}^1T_{b,k} Y^{2,*}_{i,\epsilon} Z^*_{\epsilon,\gamma} Y^{3,*}_{b,\gamma} Y^{4,*}_{j,\gamma} {}^2D^{a,i,b,j} {}^2T_{c,i,a,l} V_{l,c,k,j} \quad (1051)$$

Factorized expression

$$\tau^0_{\gamma,\alpha,w} = \sum_{a \in V} {}^2D^3_{a,w} W^1_{a,\alpha} Y^{3,*}_{a,\gamma} \quad (3r_D r_T r_V N_v) \quad (1052)$$

$$\tau^1_{\gamma,\alpha} = \sum_{a \in V} W^2_{a,\alpha} Y^1_{a,\gamma} \quad (2r_T r_V N_v) \quad (1053)$$

$$\tau^2_{\gamma,\alpha,i} = \sum_{\delta \in A} Y^2_{i,\delta} Z_{\delta,\gamma} \tau^1_{\delta,\alpha} \quad (3r_T^2 r_V N_o) \quad (1054)$$

$$\tau^3_{\gamma,\delta,\alpha,w} = \sum_{i \in O} {}^2D^4_{i,w} Y^{4,*}_{i,\delta} \tau^0_{\delta,\alpha,w} \tau^2_{\gamma,\alpha,i} \quad (4r_D r_T^2 r_V N_o) \quad (1055)$$

$$\tau^4_{\alpha,i} = \sum_{a \in V} {}^1T_{a,i} W^4_{a,\alpha} \quad (2r_V N_o N_v) \quad (1056)$$

$$\tau^5_{\alpha,i,j} = \sum_{\beta \in B} X_{\alpha,\beta} W^3_{j,\beta} \tau^4_{\beta,i} \quad (3r_V^2 N_o^2) \quad (1057)$$

$$\tau^6_{\gamma,\alpha,i} = \sum_{j \in O} Y^4_{j,\gamma} \tau^5_{\alpha,i,j} \quad (2r_T r_V N_o^2) \quad (1058)$$

$$\tau^7_{\gamma,\delta,w,i} = \sum_{\alpha \in B} \tau^6_{\gamma,\alpha,i} \tau^3_{\gamma,\delta,\alpha,w} \quad (2r_D r_T^2 r_V N_o) \quad (1059)$$

$$\tau^8_{\gamma,\delta,w} = \sum_{\epsilon \in A} \sum_{i \in O} {}^2D^2_{i,w} Y^{2,*}_{i,\delta} Z^*_{\delta,\epsilon} \tau^7_{\gamma,\epsilon,w,i} \quad (4r_D r_T^3 N_o) \quad (1060)$$

$${}^{21}R_{a,\gamma} \leftarrow - \sum_{\delta \in A} \sum_{w \in D} \frac{1}{2} D^1_{a,w} Y^3_{a,\delta} \tau^8_{\delta,\gamma,w} \quad (3r_D r_T^2 N_v) \quad (1061)$$

Raw expression

$${}^{21}R_{a,\epsilon} \leftarrow \sum_{\gamma \in A} \sum_{i \in O} \sum_{j \in O} \sum_{k \in O} \sum_{l \in O} \sum_{b \in V} \sum_{c \in V} \frac{1}{2} {}^1T_{b,k} Y^{2,*}_{i,\epsilon} Z^*_{\epsilon,\gamma} Y^{3,*}_{b,\gamma} Y^{4,*}_{j,\gamma} {}^2D^{a,i,b,j} {}^2T_{c,j,a,l} V_{l,i,k,c} \quad (1062)$$

Factorized expression

$$\tau^0_{\gamma,\alpha} = \sum_{a \in V} W^2_{a,\alpha} Y^3_{a,\gamma} \quad (2r_T r_V N_v) \quad (1063)$$

$$\tau^1_{\gamma,\alpha,i} = \sum_{\delta \in A} Z_{\gamma,\delta} Y^4_{i,\delta} \tau^0_{\delta,\alpha} \quad (3r_T^2 r_V N_o) \quad (1064)$$

$$\tau^2_{\gamma,\delta,w} = \sum_{a \in V} {}^2D^3_{a,w} Y^1_{a,\gamma} Y^{3,*}_{a,\delta} \quad (3r_D r_T^2 N_v) \quad (1065)$$

$$\tau^3_{\gamma,\delta,w,i} = \sum_{\epsilon \in A} {}^2D^4_{i,w} Z^*_{\delta,\epsilon} Y^{4,*}_{i,\epsilon} \tau^2_{\gamma,\epsilon,w} \quad (4r_D r_T^3 N_o) \quad (1066)$$

$$\tau^4_{\alpha,i} = \sum_{a \in V} {}^1T_{a,i} W^4_{a,\alpha} \quad (2r_V N_o N_v) \quad (1067)$$

$$\tau^5_{\alpha,i,j} = \sum_{\beta \in B} X_{\alpha,\beta} W^3_{j,\beta} \tau^4_{\beta,i} \quad (3r_V^2 N_o^2) \quad (1068)$$

$$\tau^6_{\gamma,\alpha,i} = \sum_{j \in O} Y^2_{j,\gamma} \tau^5_{\alpha,i,j} \quad (2r_T r_V N_o^2) \quad (1069)$$

$$\tau^7_{\gamma,\delta,\alpha,w} = \sum_{i \in O} \tau^6_{\gamma,\alpha,i} \tau^3_{\gamma,\delta,w,i} \quad (2r_D r_T^2 r_V N_o) \quad (1070)$$

$$\tau^8_{\gamma,\alpha,w,i} = \sum_{\delta \in A} \tau^1_{\delta,\alpha,i} \tau^7_{\delta,\gamma,\alpha,w} \quad (2r_D r_T^2 r_V N_o) \quad (1071)$$

$$\tau^8_{\gamma,\alpha,w,i} = \sum_{\delta \in A} \tau^1_{\delta,\alpha,i} \tau^7_{\delta,\gamma,\alpha,w} \quad (2r_D r_T^2 r_V N_o) \quad (1084)$$

$$\tau^9_{\gamma,\alpha,w} = \sum_{i \in O} {}^2D^2_{i,w} Y^{2,*}_{i,\gamma} \tau^8_{\gamma,\alpha,w,i} \quad (3r_D r_T r_V N_o) \quad (1072)$$

$$\tau^9_{\gamma,\alpha,w} = \sum_{i \in O} {}^2D^2_{i,w} Y^{2,*}_{i,\gamma} \tau^8_{\gamma,\alpha,w,i} \quad (3r_D r_T r_V N_o) \quad (1085)$$

$$\tau^{10}_{\gamma,w,a} = \sum_{\alpha \in B} W^1_{a,\alpha} \tau^9_{\gamma,\alpha,w} \quad (2r_D r_T r_V N_v) \quad (1073)$$

$$\tau^{10}_{\gamma,w,a} = \sum_{\alpha \in B} W^1_{a,\alpha} \tau^9_{\gamma,\alpha,w} \quad (2r_D r_T r_V N_v) \quad (1086)$$

$${}^{21}R_{a,\gamma} \leftarrow - \sum_{w \in D} \frac{1}{2} {}^2D^1_{a,w} \tau^{10}_{\gamma,w,a} \quad (2r_D r_T N_v) \quad (1074)$$

$${}^{21}R_{a,\gamma} \leftarrow - \sum_{w \in D} \frac{1}{2} {}^2D^1_{a,w} \tau^{10}_{\gamma,w,a} \quad (2r_D r_T N_v) \quad (1087)$$

Raw expression

$${}^{21}R_{a,\epsilon} \leftarrow \sum_{\gamma \in A} \sum_{i \in O} \sum_{j \in O} \sum_{k \in O} \sum_{l \in O} \sum_{b \in V} \sum_{c \in V} \frac{1}{2} {}^1T_{b,k} Y^{2,*}_{i,\epsilon} Z^*_{\epsilon,\gamma} Y^{3,*}_{b,\gamma} Y^{4,*}_{j,\gamma} {}^2D^{a,i,b,j} {}^2T_{c,l,a,i} V_{k,c,l,j} \quad (1075)$$

Raw expression

$${}^{21}R_{a,\epsilon} \leftarrow \sum_{\gamma \in A} \sum_{i \in O} \sum_{j \in O} \sum_{k \in O} \sum_{l \in O} \sum_{b \in V} \sum_{c \in V} \frac{1}{2} {}^1T_{c,i} Y^{2,*}_{i,\epsilon} Z^*_{\epsilon,\gamma} Y^{3,*}_{b,\gamma} Y^{4,*}_{j,\gamma} {}^2D^{a,i,b,j} {}^2T_{a,k,b,l} V_{k,c,l,j} \quad (1088)$$

Factorized expression

$$\tau^0_{\gamma,\alpha} = \sum_{a \in V} W^2_{a,\alpha} Y^1_{a,\gamma} \quad (2r_T r_V N_v) \quad (1076)$$

$$\tau^0_{\gamma,\alpha} = \sum_{i \in O} W^3_{i,\alpha} Y^2_{i,\gamma} \quad (2r_T r_V N_o) \quad (1089)$$

$$\tau^1_{\gamma,\alpha,i} = \sum_{\delta \in A} Y^2_{i,\delta} Z_{\delta,\gamma} \tau^0_{\delta,\alpha} \quad (3r_T^2 r_V N_o) \quad (1077)$$

$$\tau^1_{\gamma,\alpha} = \sum_{a \in V} W^4_{a,\alpha} Y^3_{a,\gamma} \quad (2r_T r_V N_v) \quad (1090)$$

$$\tau^2_{\gamma,\delta,w} = \sum_{a \in V} {}^2D^3_{a,w} Y^3_{a,\gamma} Y^{3,*}_{a,\delta} \quad (3r_D r_T^2 N_v) \quad (1078)$$

$$\tau^2_{\gamma,\alpha,i} = \sum_{\delta \in A} Z_{\gamma,\delta} Y^4_{i,\delta} \tau^1_{\delta,\alpha} \quad (3r_T^2 r_V N_o) \quad (1091)$$

$$\tau^3_{\gamma,\delta,w,i} = \sum_{\epsilon \in A} {}^2D^4_{i,w} Z^*_{\delta,\epsilon} Y^{4,*}_{i,\epsilon} \tau^2_{\gamma,\epsilon,w} \quad (4r_D r_T^3 N_o) \quad (1079)$$

$$\tau^3_{\alpha,i} = \sum_{a \in V} {}^1T_{a,i} W^2_{a,\alpha} \quad (2r_V N_o N_v) \quad (1092)$$

$$\tau^4_{\alpha,i} = \sum_{a \in V} {}^1T_{a,i} W^4_{a,\alpha} \quad (2r_V N_o N_v) \quad (1080)$$

$$\tau^4_{\gamma,\alpha,w} = \sum_{i \in O} {}^2D^4_{i,w} Y^{4,*}_{i,\gamma} \tau^3_{\alpha,i} \quad (3r_D r_T r_V N_o) \quad (1093)$$

$$\tau^5_{\alpha,i,j} = \sum_{\beta \in B} X_{\alpha,\beta} W^3_{j,\beta} \tau^4_{\beta,i} \quad (3r_V^2 N_o^2) \quad (1081)$$

$$\tau^5_{\gamma,\alpha,w} = \sum_{a \in V} {}^2D^3_{a,w} W^1_{a,\alpha} Y^{3,*}_{a,\gamma} \quad (3r_D r_T r_V N_v) \quad (1094)$$

$$\tau^6_{\gamma,\alpha,i} = \sum_{j \in O} Y^4_{j,\gamma} \tau^5_{\alpha,i,j} \quad (2r_T r_V N_o^2) \quad (1082)$$

$$\tau^6_{\gamma,\alpha,w} = \sum_{\beta \in B} X_{\beta,\alpha} \tau^4_{\gamma,\beta,w} \tau^5_{\gamma,\beta,w} \quad (3r_D r_T r_V^2) \quad (1095)$$

$$\tau^7_{\gamma,\delta,\alpha,w} = \sum_{i \in O} \tau^6_{\gamma,\alpha,i} \tau^3_{\gamma,\delta,w,i} \quad (2r_D r_T^2 r_V N_o) \quad (1083)$$

$$\tau^7_{\gamma,\alpha,w} = \sum_{\delta \in A} Z^*_{\gamma,\delta} \tau^6_{\delta,\alpha,w} \quad (2r_D r_T^2 r_V) \quad (1096)$$

$$\tau_{\gamma,\delta,w,i}^8 = \sum_{\alpha \in B} \tau_{\gamma,\alpha}^0 \tau_{\gamma,\alpha,i}^2 \tau_{\delta,\alpha,w}^7 \quad (3r_D r_T^2 r_V N_o) \quad (1097)$$

$$\tau_{\gamma,\delta,w,i}^8 = \sum_{\alpha \in B} \tau_{\gamma,\alpha}^2 \tau_{\gamma,\alpha,i}^1 \tau_{\delta,\alpha,w}^7 \quad (3r_D r_T^2 r_V N_o) \quad (1109)$$

$$\tau_{\gamma,\delta,w}^9 = \sum_{i \in O} {}^2D_{i,w}^2 Y_{i,\delta}^{2,*} \tau_{\gamma,\delta,w,i}^8 \quad (3r_D r_T^2 N_o) \quad (1098)$$

$$\tau_{\gamma,\delta,w}^9 = \sum_{i \in O} {}^2D_{i,w}^2 Y_{i,\delta}^{2,*} \tau_{\gamma,\delta,w,i}^8 \quad (3r_D r_T^2 N_o) \quad (1110)$$

$${}^{21}R_{a,\gamma} \leftarrow - \sum_{\delta \in A} \sum_{w \in D} \frac{1}{2} {}^2D_{a,w}^1 Y_{a,\delta}^1 \tau_{\delta,\gamma,w}^9 \quad (3r_D r_T^2 N_v) \quad (1099)$$

$${}^{21}R_{a,\gamma} \leftarrow - \sum_{\delta \in A} \sum_{w \in D} \frac{1}{2} {}^2D_{a,w}^1 Y_{a,\delta}^3 \tau_{\delta,\gamma,w}^9 \quad (3r_D r_T^2 N_v) \quad (1111)$$

Raw expression

$${}^{21}R_{a,\epsilon} \leftarrow \sum_{\gamma \in A} \sum_{i \in O} \sum_{j \in O} \sum_{k \in O} \sum_{l \in O} \sum_{b \in V} \sum_{c \in V} \frac{1}{2} {}^1T_{c,i} Y_{i,\epsilon}^{2,*} Z_{\epsilon,\gamma}^* Y_{b,\gamma}^{3,*} Y_{j,\gamma}^{4,*} {}^2D_{a,i,b,j} {}^2T_{b,k,a,l} V_{l,c,k,j} \quad (1100)$$

Raw expression

$${}^{21}R_{a,\epsilon} \leftarrow \sum_{\gamma \in A} \sum_{i \in O} \sum_{j \in O} \sum_{k \in O} \sum_{l \in O} \sum_{b \in V} \sum_{c \in V} \frac{1}{2} {}^1T_{c,j} Y_{i,\epsilon}^{2,*} Z_{\epsilon,\gamma}^* Y_{b,\gamma}^{3,*} Y_{j,\gamma}^{4,*} {}^2D_{a,i,b,j} {}^2T_{a,k,b,l} V_{k,i,l,c} \quad (1112)$$

Factorized expression

$$\tau_{\gamma,\alpha}^0 = \sum_{a \in V} W_{a,\alpha}^4 Y_{a,\gamma}^1 \quad (2r_T r_V N_v) \quad (1101)$$

$$\tau_{\gamma,\delta,w}^0 = \sum_{i \in O} {}^2D_{i,w}^2 Y_{i,\gamma}^2 Y_{i,\delta}^{2,*} \quad (3r_D r_T^2 N_o) \quad (1113)$$

$$\tau_{\gamma,\alpha,i}^1 = \sum_{\delta \in A} Y_{i,\delta}^2 Z_{\delta,\gamma} \tau_{\delta,\alpha}^0 \quad (3r_T^2 r_V N_o) \quad (1102)$$

$$\tau_{\alpha,i}^1 = \sum_{a \in V} {}^1T_{a,i} W_{a,\alpha}^4 \quad (2r_V N_o N_v) \quad (1114)$$

$$\tau_{\gamma,\alpha}^2 = \sum_{i \in O} W_{i,\alpha}^3 Y_{i,\gamma}^4 \quad (2r_T r_V N_o) \quad (1103)$$

$$\tau_{\alpha,i,j}^2 = \sum_{\beta \in B} X_{\alpha,\beta} W_{j,\beta}^3 \tau_{\beta,i}^1 \quad (3r_V^2 N_o^2) \quad (1115)$$

$$\tau_{\alpha,i}^3 = \sum_{a \in V} {}^1T_{a,i} W_{a,\alpha}^2 \quad (2r_V N_o N_v) \quad (1104)$$

$$\tau_{\gamma,\alpha,i}^3 = \sum_{j \in O} Y_{j,\gamma}^4 \tau_{\alpha,i,j}^2 \quad (2r_T r_V N_o^2) \quad (1116)$$

$$\tau_{\gamma,\alpha,w}^4 = \sum_{i \in O} {}^2D_{i,w}^4 Y_{i,\gamma}^{4,*} \tau_{\alpha,i}^3 \quad (3r_D r_T r_V N_o) \quad (1105)$$

$$\tau_{\gamma,\alpha}^4 = \sum_{a \in V} W_{a,\alpha}^2 Y_{a,\gamma}^3 \quad (2r_T r_V N_v) \quad (1117)$$

$$\tau_{\gamma,\alpha,w}^5 = \sum_{a \in V} {}^2D_{a,w}^3 W_{a,\alpha}^1 Y_{a,\gamma}^{3,*} \quad (3r_D r_T r_V N_v) \quad (1106)$$

$$\tau_{\gamma,i,a}^5 = \sum_{\alpha \in B} W_{a,\alpha}^1 \tau_{\gamma,\alpha}^4 \tau_{\gamma,\alpha,i}^3 \quad (3r_T r_V N_o N_v) \quad (1118)$$

$$\tau_{\gamma,\alpha,w}^6 = \sum_{\beta \in B} X_{\beta,\alpha} \tau_{\gamma,\beta,w}^4 \tau_{\gamma,\beta,w}^5 \quad (3r_D r_T r_V^2) \quad (1107)$$

$$\tau_{\gamma,\delta,w}^6 = \sum_{i \in O} \sum_{a \in V} {}^2D_{a,w}^3 {}^2D_{i,w}^4 Y_{a,\delta}^{3,*} Y_{i,\delta}^{4,*} \tau_{\gamma,i,a}^5 \quad (5r_D r_T^2 N_o N_v) \quad (1119)$$

$$\tau_{\gamma,\alpha,w}^7 = \sum_{\delta \in A} Z_{\gamma,\delta}^* \tau_{\delta,\alpha,w}^6 \quad (2r_D r_T^2 r_V) \quad (1108)$$

$$\tau_{\gamma,\delta,w}^7 = \sum_{\epsilon \in A} Z_{\delta,\epsilon}^* \tau_{\gamma,\epsilon,w}^6 \quad (2r_D r_T^3) \quad (1120)$$

Raw expression

$$\tau_{\gamma,\delta,w}^8 = \sum_{\epsilon \in A} Z_{\gamma,\epsilon} \tau_{\epsilon,\delta,w}^7 \quad (2r_D r_T^3) \quad (1121)$$

$${}^{21}R_{a,\gamma} \leftarrow - \sum_{\delta \in A} \sum_{w \in D} \frac{1}{2} D_{a,w}^1 Y_{a,\delta}^1 \tau_{\delta,\gamma,w}^0 \tau_{\delta,\gamma,w}^8 \quad (4r_D r_T^2 N_v) \quad (1122)$$

Raw expression

$${}^{21}R_{a,\epsilon} \leftarrow \sum_{\gamma \in A} \sum_{i \in O} \sum_{j \in O} \sum_{k \in O} \sum_{l \in O} \sum_{b \in V} \sum_{c \in V} \frac{1}{2} {}^1T_{c,j} Y_{i,\epsilon}^{2,*} Z_{\epsilon,\gamma}^* Y_{b,\gamma}^{3,*} Y_{j,\gamma}^{4,*} {}^2D_{a,i,b,j} {}^2T_{b,k,a,l} V_{l,i,k,c} \quad (1123)$$

Factorized expression

$$\tau_{\gamma,\delta,w}^0 = \sum_{i \in O} {}^2D_{i,w}^2 Y_{i,\gamma}^4 Y_{i,\delta}^{2,*} \quad (3r_D r_T^2 N_o) \quad (1124)$$

$$\tau_{\alpha,i}^1 = \sum_{a \in V} {}^1T_{a,i} W_{a,\alpha}^4 \quad (2r_V N_o N_v) \quad (1125)$$

$$\tau_{\alpha,i,j}^2 = \sum_{\beta \in B} X_{\alpha,\beta} W_{j,\beta}^3 \tau_{\beta,i}^1 \quad (3r_V^2 N_o^2) \quad (1126)$$

$$\tau_{\gamma,\alpha,i}^3 = \sum_{j \in O} Y_{j,\gamma}^2 \tau_{\alpha,i,j}^2 \quad (2r_T r_V N_o^2) \quad (1127)$$

$$\tau_{\gamma,\alpha}^4 = \sum_{a \in V} W_{a,\alpha}^2 Y_{a,\gamma}^1 \quad (2r_T r_V N_v) \quad (1128)$$

$$\tau_{\gamma,i,a}^5 = \sum_{\alpha \in B} W_{a,\alpha}^1 \tau_{\gamma,\alpha}^4 \tau_{\gamma,\alpha,i}^3 \quad (3r_T r_V N_o N_v) \quad (1129)$$

$$\tau_{\gamma,\delta,w}^6 = \sum_{i \in O} \sum_{a \in V} {}^2D_{a,w}^3 {}^2D_{i,w}^4 Y_{a,\delta}^{3,*} Y_{i,\delta}^{4,*} \tau_{\gamma,i,a}^5 \quad (5r_D r_T^2 N_o N_v) \quad (1130)$$

$$\tau_{\gamma,\delta,w}^7 = \sum_{\epsilon \in A} Z_{\delta,\epsilon}^* \tau_{\gamma,\epsilon,w}^6 \quad (2r_D r_T^3) \quad (1131)$$

$$\tau_{\gamma,\delta,w}^8 = \sum_{\epsilon \in A} Z_{\epsilon,\gamma} \tau_{\epsilon,\delta,w}^7 \quad (2r_D r_T^3) \quad (1132)$$

$${}^{21}R_{a,\gamma} \leftarrow - \sum_{\delta \in A} \sum_{w \in D} \frac{1}{2} D_{a,w}^1 Y_{a,\delta}^3 \tau_{\delta,\gamma,w}^0 \tau_{\delta,\gamma,w}^8 \quad (4r_D r_T^2 N_v) \quad (1133)$$

$${}^{21}R_{a,\epsilon} \leftarrow \sum_{\gamma \in A} \sum_{i \in O} \sum_{j \in O} \sum_{k \in O} \sum_{l \in O} \sum_{b \in V} \sum_{c \in V} \frac{1}{2} {}^1T_{c,k} Y_{i,\epsilon}^{2,*} Z_{\epsilon,\gamma}^* Y_{b,\gamma}^{3,*} Y_{j,\gamma}^{4,*} {}^2D_{a,i,b,j} {}^2T_{a,i,b,l} V_{l,c,k,j} \quad (1134)$$

Factorized expression

$$\tau_{\alpha,i}^0 = \sum_{a \in V} {}^1T_{a,i} W_{a,\alpha}^2 \quad (2r_V N_o N_v) \quad (1135)$$

$$\tau_{\alpha,\beta}^1 = \sum_{i \in O} W_{i,\beta}^3 \tau_{\alpha,i}^0 \quad (2r_V^2 N_o) \quad (1136)$$

$$\tau_{\alpha,a}^2 = \sum_{\beta \in B} X_{\alpha,\beta} W_{a,\beta}^4 \tau_{\alpha,\beta}^1 \quad (3r_V^2 N_v) \quad (1137)$$

$$\tau_{a,b}^3 = \sum_{\alpha \in B} W_{a,\alpha}^1 \tau_{\alpha,b}^2 \quad (2r_V N_v^2) \quad (1138)$$

$$\tau_{\gamma,a}^4 = \sum_{b \in V} Y_{b,\gamma}^3 \tau_{a,b}^3 \quad (2r_T N_v^2) \quad (1139)$$

$$\tau_{\gamma,\delta,w}^5 = \sum_{a \in V} {}^2D_{a,w}^3 Y_{a,\gamma}^1 Y_{a,\delta}^{3,*} \quad (3r_D r_T^2 N_v) \quad (1140)$$

$$\tau_{\gamma,\delta,w}^6 = \sum_{i \in O} {}^2D_{i,w}^4 Y_{i,\gamma}^2 Y_{i,\delta}^{4,*} \quad (3r_D r_T^2 N_o) \quad (1141)$$

$$\tau_{\gamma,\delta,w}^7 = \sum_{\epsilon \in A} Z_{\delta,\epsilon}^* \tau_{\gamma,\epsilon,w}^5 \tau_{\gamma,\epsilon,w}^6 \quad (3r_D r_T^3) \quad (1142)$$

$$\tau_{\gamma,\delta,w}^8 = \sum_{\epsilon \in A} Z_{\epsilon,\gamma} \tau_{\epsilon,\delta,w}^7 \quad (2r_D r_T^3) \quad (1143)$$

$$\tau_{\gamma,\delta,w}^9 = \sum_{i \in O} {}^2D_{i,w}^2 Y_{i,\gamma}^4 Y_{i,\delta}^{2,*} \quad (3r_D r_T^2 N_o) \quad (1144)$$

$${}^{21}R_{a,\gamma} \leftarrow - \sum_{\delta \in A} \sum_{w \in D} \frac{1}{2} D_{a,w}^1 \tau_{\delta,a}^4 \tau_{\delta,\gamma,w}^8 \tau_{\delta,\gamma,w}^9 \quad (4r_D r_T^2 N_v) \quad (1145)$$

Raw expression

$${}^{21}R_{a,\epsilon} \leftarrow \sum_{\gamma \in A} \sum_{i \in O} \sum_{j \in O} \sum_{k \in O} \sum_{l \in O} \sum_{b \in V} \sum_{c \in V} \frac{1}{2} {}^1T_{c,k} Y_{i,\epsilon}^{2,*} Z_{\epsilon,\gamma}^* Y_{b,\gamma}^{3,*} Y_{j,\gamma}^{4,*} {}^2D_{a,i,b,j} {}^2T_{a,i,b,j} V_{k,i,l,c} \quad (1146)$$

Factorized expression

$$\tau^0_{\alpha,i} = \sum_{a \in V} {}^1T_{a,i} W^2_{a,\alpha} \quad (2r_V N_o N_v) \quad (1147)$$

$$\tau^1_{\alpha,\beta} = \sum_{i \in O} W^3_{i,\beta} \tau^0_{\alpha,i} \quad (2r_V^2 N_o) \quad (1148)$$

$$\tau^2_{\alpha,a} = \sum_{\beta \in B} X_{\alpha,\beta} W^4_{a,\beta} \tau^1_{\alpha,\beta} \quad (3r_V^2 N_v) \quad (1149)$$

$$\tau^3_{a,b} = \sum_{\alpha \in B} W^1_{a,\alpha} \tau^2_{\alpha,b} \quad (2r_V N_v^2) \quad (1150)$$

$$\tau^4_{\gamma,a} = \sum_{b \in V} Y^1_{b,\gamma} \tau^3_{a,b} \quad (2r_T N_v^2) \quad (1151)$$

$$\tau^5_{\gamma,\delta,w} = \sum_{i \in O} {}^2D^2_{i,w} Y^2_{i,\gamma} Y^{2,*}_{i,\delta} \quad (3r_D r_T^2 N_o) \quad (1152)$$

$$\tau^6_{\gamma,\delta,w} = \sum_{a \in V} {}^2D^3_{a,w} Y^3_{a,\gamma} Y^{3,*}_{a,\delta} \quad (3r_D r_T^2 N_v) \quad (1153)$$

$$\tau^7_{\gamma,\delta,w} = \sum_{i \in O} {}^2D^4_{i,w} Y^4_{i,\gamma} Y^{4,*}_{i,\delta} \quad (3r_D r_T^2 N_o) \quad (1154)$$

$$\tau^8_{\gamma,\delta,w} = \sum_{\epsilon \in A} Z^*_{\delta,\epsilon} \tau^6_{\gamma,\epsilon,w} \tau^7_{\gamma,\epsilon,w} \quad (3r_D r_T^3) \quad (1155)$$

$$\tau^9_{\gamma,\delta,w} = \sum_{\epsilon \in A} Z_{\gamma,\epsilon} \tau^8_{\epsilon,\delta,w} \quad (2r_D r_T^3) \quad (1156)$$

$${}^{21}R_{a,\gamma} \leftarrow - \sum_{\delta \in A} \sum_{w \in D} \frac{1}{2} {}^2D^1_{a,w} \tau^4_{\delta,a} \tau^5_{\delta,\gamma,w} \tau^9_{\delta,\gamma,w} \quad (4r_D r_T^2 N_v) \quad \text{Raw expression} \quad (1157)$$

Raw expression

$${}^{21}R_{a,\epsilon} \leftarrow \sum_{\gamma \in A} \sum_{i \in O} \sum_{j \in O} \sum_{k \in O} \sum_{l \in O} \sum_{b \in V} \sum_{c \in V} \frac{1}{2} {}^1T_{c,k} Y^{2,*}_{i,\epsilon} Z^*_{\epsilon,\gamma} Y^{3,*}_{b,\gamma} Y^{4,*}_{j,\gamma} {}^2D^{a,i,b,j} {}^2T_{b,j,a,l} V_{k,i,l,c} \quad (1158)$$

Factorized expression

$$\tau^0_{\gamma,\delta,w} = \sum_{i \in O} {}^2D^2_{i,w} Y^2_{i,\gamma} Y^{2,*}_{i,\delta} \quad (3r_D r_T^2 N_o) \quad (1159)$$

$$\tau^1_{\gamma,\delta,w} = \sum_{i \in O} {}^2D^4_{i,w} Y^4_{i,\gamma} Y^{4,*}_{i,\delta} \quad (3r_D r_T^2 N_o) \quad (1160)$$

$$\tau^2_{\alpha,i} = \sum_{a \in V} {}^1T_{a,i} W^2_{a,\alpha} \quad (2r_V N_o N_v) \quad (1161)$$

$$\tau^3_{\alpha,\beta} = \sum_{i \in O} W^3_{i,\beta} \tau^2_{\alpha,i} \quad (2r_V^2 N_o) \quad (1162)$$

$$\tau^4_{\alpha,a} = \sum_{\beta \in B} X_{\alpha,\beta} W^4_{a,\beta} \tau^3_{\alpha,\beta} \quad (3r_V^2 N_v) \quad (1163)$$

$$\tau^5_{a,b} = \sum_{\alpha \in B} W^1_{a,\alpha} \tau^4_{\alpha,b} \quad (2r_V N_v^2) \quad (1164)$$

$$\tau^6_{\gamma,a} = \sum_{b \in V} Y^3_{b,\gamma} \tau^5_{a,b} \quad (2r_T N_v^2) \quad (1165)$$

$$\tau^7_{\gamma,\delta,w} = \sum_{a \in V} {}^2D^3_{a,w} Y^{3,*}_{a,\delta} \tau^6_{\gamma,a} \quad (3r_D r_T^2 N_v) \quad (1166)$$

$$\tau^8_{\gamma,\delta,w} = \sum_{\epsilon \in A} Z^*_{\delta,\epsilon} \tau^1_{\gamma,\epsilon,w} \tau^7_{\gamma,\epsilon,w} \quad (3r_D r_T^3) \quad (1167)$$

$$\tau^9_{\gamma,\delta,w} = \sum_{\epsilon \in A} Z_{\gamma,\epsilon} \tau^8_{\epsilon,\delta,w} \quad (2r_D r_T^3) \quad (1168)$$

$${}^{21}R_{a,\gamma} \leftarrow - \sum_{\delta \in A} \sum_{w \in D} \frac{1}{2} {}^2D^1_{a,w} Y^1_{a,\delta} \tau^0_{\delta,\gamma,w} \tau^9_{\delta,\gamma,w} \quad (4r_D r_T^2 N_v) \quad (1169)$$

$${}^{21}R_{a,\epsilon} \leftarrow \sum_{\gamma \in A} \sum_{i \in O} \sum_{j \in O} \sum_{k \in O} \sum_{l \in O} \sum_{b \in V} \sum_{c \in V} \frac{1}{2} {}^1T_{c,k} Y^{2,*}_{i,\epsilon} Z^*_{\epsilon,\gamma} Y^{3,*}_{b,\gamma} Y^{4,*}_{j,\gamma} {}^2D^{a,i,b,j} {}^2T_{b,l,a,i} V_{l,c,k,j} \quad (1170)$$

Factorized expression

$$\tau^0_{\gamma,\delta,w} = \sum_{i \in O} {}^2D^4_{i,w} Y^2_{i,\gamma} Y^{4,*}_{i,\delta} \quad (3r_D r_T^2 N_o) \quad (1171)$$

$$\tau^1_{\alpha,i} = \sum_{a \in V} {}^1T_{a,i} W^2_{a,\alpha} \quad (2r_V N_o N_v) \quad (1172)$$

$$\tau^2_{\alpha,\beta} = \sum_{i \in O} W^3_{i,\beta} \tau^1_{\alpha,i} \quad (2r_V^2 N_o) \quad (1173)$$

$$\tau^3_{\gamma,\alpha} = \sum_{\beta \in B} X_{\alpha,\beta} \tau^1_{\gamma,\beta} \tau^2_{\gamma,\beta} \quad (3r_T r_V^2) \quad (1186)$$

$$\tau^3_{\alpha,a} = \sum_{\beta \in B} X_{\alpha,\beta} W^4_{a,\beta} \tau^2_{\alpha,\beta} \quad (3r_V^2 N_v) \quad (1174)$$

$$\tau^4_{\gamma,\alpha} = \sum_{\delta \in A} Z_{\gamma,\delta} \tau^3_{\delta,\alpha} \quad (2r_T^2 r_V) \quad (1187)$$

$$\tau^4_{a,b} = \sum_{\alpha \in B} W^1_{a,\alpha} \tau^3_{\alpha,b} \quad (2r_V N_v^2) \quad (1175)$$

$$\tau^5_{\gamma,\delta,w} = \sum_{a \in V} {}^2D^3_{a,w} Y^1_{a,\gamma} Y^{3,*}_{a,\delta} \quad (3r_D r_T^2 N_v) \quad (1188)$$

$$\tau^5_{\gamma,a} = \sum_{b \in V} Y^1_{b,\gamma} \tau^4_{a,b} \quad (2r_T N_v^2) \quad (1176)$$

$$\tau^6_{\gamma,\delta,w} = \sum_{i \in O} {}^2D^4_{i,w} Y^2_{i,\gamma} Y^{4,*}_{i,\delta} \quad (3r_D r_T^2 N_o) \quad (1189)$$

$$\tau^6_{\gamma,\delta,w} = \sum_{a \in V} {}^2D^3_{a,w} Y^{3,*}_{a,\delta} \tau^5_{\gamma,a} \quad (3r_D r_T^2 N_v) \quad (1177)$$

$$\tau^7_{\gamma,\delta,w} = \sum_{\epsilon \in A} Z^*_{\delta,\epsilon} \tau^5_{\gamma,\epsilon,w} \tau^6_{\gamma,\epsilon,w} \quad (3r_D r_T^3) \quad (1190)$$

$$\tau^7_{\gamma,\delta,w} = \sum_{\epsilon \in A} Z^*_{\delta,\epsilon} \tau^0_{\gamma,\epsilon,w} \tau^6_{\gamma,\epsilon,w} \quad (3r_D r_T^3) \quad (1178)$$

$$\tau^8_{\gamma,\alpha,w} = \sum_{\delta \in A} \tau^4_{\delta,\alpha} \tau^7_{\delta,\gamma,w} \quad (2r_D r_T^2 r_V) \quad (1191)$$

$$\tau^8_{\gamma,\delta,w} = \sum_{\epsilon \in A} Z_{\epsilon,\gamma} \tau^7_{\epsilon,\delta,w} \quad (2r_D r_T^3) \quad (1179)$$

$$\tau^9_{\gamma,w,i} = \sum_{\alpha \in B} W^1_{i,\alpha} \tau^0_{\gamma,\alpha,w} \tau^8_{\gamma,\alpha,w} \quad (3r_D r_T r_V N_o) \quad (1192)$$

$$\tau^9_{\gamma,\delta,w} = \sum_{i \in O} {}^2D^2_{i,w} Y^4_{i,\gamma} Y^{2,*}_{i,\delta} \quad (3r_D r_T^2 N_o) \quad (1180)$$

$${}^{21}R_{a,\gamma} \leftarrow - \sum_{w \in D} \sum_{i \in O} {}^2D^1_{a,w} {}^1T_{a,i} \tau^9_{\gamma,w,i} \quad (3r_D r_T N_o N_v) \quad (1193)$$

$${}^{21}R_{a,\gamma} \leftarrow - \sum_{\delta \in A} \sum_{w \in D} \frac{1}{2} {}^2D^1_{a,w} Y^3_{a,\delta} \tau^8_{\delta,\gamma,w} \tau^9_{\delta,\gamma,w} \quad (4r_D r_T^2 N_v) \text{Raw expression} \quad (1181)$$

Raw expression

$${}^{21}R_{a,\epsilon} \leftarrow - \sum_{\gamma \in A} \sum_{i \in O} \sum_{j \in O} \sum_{k \in O} \sum_{l \in O} \sum_{b \in V} \sum_{c \in V} {}^1T_{a,k} Y^{2,*}_{i,\epsilon} Z^*_{\epsilon,\gamma} Y^{3,*}_{b,\gamma} Y^{4,*}_{j,\gamma} {}^2D^{a,i,b,j} {}^2T_{b,j,c,l} V_{k,i,l,c} \quad (1182)$$

Factorized expression

$$\tau^0_{\gamma,\alpha,w} = \sum_{i \in O} {}^2D^2_{i,w} W^2_{i,\alpha} Y^{2,*}_{i,\gamma} \quad (3r_D r_T r_V N_o) \quad (1183)$$

$$\tau^1_{\gamma,\alpha} = \sum_{a \in V} W^4_{a,\alpha} Y^3_{a,\gamma} \quad (2r_T r_V N_v) \quad (1184)$$

$$\tau^2_{\gamma,\alpha} = \sum_{i \in O} W^3_{i,\alpha} Y^4_{i,\gamma} \quad (2r_T r_V N_o) \quad (1185)$$

$${}^{21}R_{a,\epsilon} \leftarrow - \sum_{\gamma \in A} \sum_{i \in O} \sum_{j \in O} \sum_{k \in O} \sum_{l \in O} \sum_{b \in V} \sum_{c \in V} {}^1T_{a,k} Y^{2,*}_{i,\epsilon} Z^*_{\epsilon,\gamma} Y^{3,*}_{b,\gamma} Y^{4,*}_{j,\gamma} {}^2D^{a,i,b,j} {}^2T_{c,l,b,j} V_{k,i,l,c} \quad (1194)$$

Factorized expression

$$\tau^0_{\gamma,\alpha,w} = \sum_{i \in O} {}^2D^2_{i,w} W^2_{i,\alpha} Y^{2,*}_{i,\gamma} \quad (3r_D r_T r_V N_o) \quad (1195)$$

$$\tau^1_{\gamma,\delta,w} = \sum_{a \in V} {}^2D^3_{a,w} Y^3_{a,\gamma} Y^{3,*}_{a,\delta} \quad (3r_D r_T^2 N_v) \quad (1196)$$

$$\tau^2_{\gamma,\delta,w} = \sum_{i \in O} {}^2D^4_{i,w} Y^4_{i,\gamma} Y^{4,*}_{i,\delta} \quad (3r_D r_T^2 N_o) \quad (1197)$$

$$\tau^3_{\gamma,\delta,w} = \sum_{\epsilon \in A} Z^*_{\delta,\epsilon} \tau^1_{\gamma,\epsilon,w} \tau^2_{\gamma,\epsilon,w} \quad (3r_D r_T^3) \quad (1198)$$



$$\tau^4_{\gamma,\alpha} = \sum_{a \in V} W^4_{a,\alpha} Y^1_{a,\gamma} \quad (2r_T r_V N_v) \quad (1199)$$

$$\tau^5_{\gamma,\alpha} = \sum_{i \in O} W^3_{i,\alpha} Y^2_{i,\gamma} \quad (2r_T r_V N_o) \quad (1200)$$

$$\tau^6_{\gamma,\alpha} = \sum_{\beta \in B} X_{\alpha,\beta} \tau^4_{\gamma,\beta} \tau^5_{\gamma,\beta} \quad (3r_T r_V^2) \quad (1201)$$

$$\tau^7_{\gamma,\alpha} = \sum_{\delta \in A} Z_{\delta,\gamma} \tau^6_{\delta,\alpha} \quad (2r_T^2 r_V) \quad (1202)$$

$$\tau^8_{\gamma,\alpha,w} = \sum_{\delta \in A} \tau^7_{\delta,\alpha} \tau^3_{\delta,\gamma,w} \quad (2r_D r_T^2 r_V) \quad (1203)$$

$$\tau^9_{\gamma,w,i} = \sum_{\alpha \in B} W^1_{i,\alpha} \tau^0_{\gamma,\alpha,w} \tau^8_{\gamma,\alpha,w} \quad (3r_D r_T r_V N_o) \quad (1204)$$

$${}^{21}R_{a,\gamma} \leftarrow - \sum_{w \in D} \sum_{i \in O} {}^2D^1_{a,w} {}^1T_{a,i} \tau^9_{\gamma,w,i} \quad (3r_D r_T N_o N_v) \quad (1205)$$

Raw expression

$${}^{21}R_{a,\epsilon} \leftarrow - \sum_{\gamma \in A} \sum_{i \in O} \sum_{j \in O} \sum_{k \in O} \sum_{l \in O} \sum_{b \in V} \sum_{c \in V} {}^1T_{b,k} Y^{2,*}_{i,\epsilon} Z^*_{\epsilon,\gamma} Y^{3,*}_{b,\gamma} Y^{4,*}_{j,\gamma} {}^2D^{a,i,b,j} {}^2T_{a,i,c,l} V_{l,c,k,j} \quad (1206)$$

Factorized expression

$$\tau^0_{\gamma,\delta,w} = \sum_{i \in O} {}^2D^2_{i,w} Y^2_{i,\gamma} Y^{2,*}_{i,\delta} \quad (3r_D r_T^2 N_o) \quad (1207)$$

$$\tau^1_{\gamma,\alpha} = \sum_{a \in V} W^2_{a,\alpha} Y^3_{a,\gamma} \quad (2r_T r_V N_v) \quad (1208)$$

$$\tau^2_{\gamma,\alpha} = \sum_{i \in O} W^1_{i,\alpha} Y^4_{i,\gamma} \quad (2r_T r_V N_o) \quad (1209)$$

$$\tau^3_{\gamma,\alpha} = \sum_{\beta \in B} X_{\beta,\alpha} \tau^1_{\gamma,\beta} \tau^2_{\gamma,\beta} \quad (3r_T r_V^2) \quad (1210)$$

$$\tau^4_{\gamma,\alpha} = \sum_{\delta \in A} Z_{\gamma,\delta} \tau^3_{\delta,\alpha} \quad (2r_T^2 r_V) \quad (1211)$$

$$\tau^5_{\gamma,w,i} = \sum_{a \in V} {}^2D^3_{a,w} {}^1T_{a,i} Y^{3,*}_{a,\gamma} \quad (3r_D r_T N_o N_v) \quad (1212)$$

$$\tau^6_{\gamma,\alpha,w} = \sum_{i \in O} W^3_{i,\alpha} \tau^5_{\gamma,w,i} \quad (2r_D r_T r_V N_o) \quad (1213)$$

$$\tau^7_{\gamma,\alpha,w} = \sum_{i \in O} {}^2D^4_{i,w} W^4_{i,\alpha} Y^{4,*}_{i,\gamma} \quad (3r_D r_T r_V N_o) \quad (1214)$$

$$\tau^8_{\gamma,\delta,w} = \sum_{\alpha \in B} \tau^4_{\gamma,\alpha} \tau^6_{\delta,\alpha,w} \tau^7_{\delta,\alpha,w} \quad (3r_D r_T^2 r_V) \quad (1215)$$

$$\tau^9_{\gamma,\delta,w} = \sum_{\epsilon \in A} Z^*_{\delta,\epsilon} \tau^8_{\gamma,\epsilon,w} \quad (2r_D r_T^3) \quad (1216)$$

$${}^{21}R_{a,\gamma} \leftarrow - \sum_{\delta \in A} \sum_{w \in D} {}^2D^1_{a,w} Y^1_{a,\delta} \tau^0_{\delta,\gamma,w} \tau^9_{\delta,\gamma,w} \quad (4r_D r_T^2 N_v) \quad (1217)$$

Raw expression

$${}^{21}R_{a,\epsilon} \leftarrow - \sum_{\gamma \in A} \sum_{i \in O} \sum_{j \in O} \sum_{k \in O} \sum_{l \in O} \sum_{b \in V} \sum_{c \in V} {}^1T_{b,k} Y^{2,*}_{i,\epsilon} Z^*_{\epsilon,\gamma} Y^{3,*}_{b,\gamma} Y^{4,*}_{j,\gamma} {}^2D^{a,i,b,j} {}^2T_{c,l,a,i} V_{l,c,k,j} \quad (1218)$$

Factorized expression

$$\tau^0_{\gamma,\delta,w} = \sum_{i \in O} {}^2D^2_{i,w} Y^4_{i,\gamma} Y^{2,*}_{i,\delta} \quad (3r_D r_T^2 N_o) \quad (1219)$$

$$\tau^1_{\gamma,\alpha} = \sum_{a \in V} W^2_{a,\alpha} Y^1_{a,\gamma} \quad (2r_T r_V N_v) \quad (1220)$$

$$\tau^2_{\gamma,\alpha} = \sum_{i \in O} W^1_{i,\alpha} Y^2_{i,\gamma} \quad (2r_T r_V N_o) \quad (1221)$$

$$\tau^3_{\gamma,\alpha} = \sum_{\beta \in B} X_{\beta,\alpha} \tau^1_{\gamma,\beta} \tau^2_{\gamma,\beta} \quad (3r_T r_V^2) \quad (1222)$$

$$\tau^4_{\gamma,\alpha} = \sum_{\delta \in A} Z_{\delta,\gamma} \tau^3_{\delta,\alpha} \quad (2r_T^2 r_V) \quad (1223)$$

$$\tau^5_{\gamma,w,i} = \sum_{a \in V} {}^2D^3_{a,w} {}^1T_{a,i} Y^{3,*}_{a,\gamma} \quad (3r_D r_T N_o N_v) \quad (1224)$$

$$\tau_{\gamma,\alpha,w}^6 = \sum_{i \in O} W_{i,\alpha}^3 \tau_{\gamma,w,i}^5 \quad (2r_D r_T r_V N_o) \quad (1225)$$

$$\tau_{\gamma,\delta,w}^7 = \sum_{i \in O} {}^2D_{i,w}^4 Y_{i,\delta}^{4,*} \tau_{\gamma,i}^6 \quad (3r_D r_T^2 N_o) \quad (1238)$$

$$\tau_{\gamma,\alpha,w}^7 = \sum_{i \in O} {}^2D_{i,w}^4 W_{i,\alpha}^4 Y_{i,\gamma}^{4,*} \quad (3r_D r_T r_V N_o) \quad (1226)$$

$$\tau_{\gamma,\delta,w}^8 = \sum_{\epsilon \in A} Z_{\delta,\epsilon}^* \tau_{\gamma,\epsilon,w}^1 \tau_{\gamma,\epsilon,w}^7 \quad (3r_D r_T^3) \quad (1239)$$

$$\tau_{\gamma,\delta,w}^8 = \sum_{\alpha \in B} \tau_{\gamma,\alpha}^4 \tau_{\delta,\alpha,w}^6 \tau_{\delta,\alpha,w}^7 \quad (3r_D r_T^2 r_V) \quad (1227)$$

$$\tau_{\gamma,\delta,w}^9 = \sum_{\epsilon \in A} Z_{\gamma,\epsilon} \tau_{\epsilon,\delta,w}^8 \quad (2r_D r_T^3) \quad (1240)$$

$$\tau_{\gamma,\delta,w}^9 = \sum_{\epsilon \in A} Z_{\delta,\epsilon}^* \tau_{\gamma,\epsilon,w}^8 \quad (2r_D r_T^3) \quad (1228)$$

$${}^{21}R_{a,\gamma} \leftarrow - \sum_{\delta \in A} \sum_{w \in D} {}^2D_{a,w}^1 Y_{a,\delta}^1 \tau_{\delta,\gamma,w}^0 \tau_{\delta,\gamma,w}^9 \quad (4r_D r_T^2 N_v) \quad (1241)$$

$${}^{21}R_{a,\gamma} \leftarrow - \sum_{\delta \in A} \sum_{w \in D} {}^2D_{a,w}^1 Y_{a,\delta}^3 \tau_{\delta,\gamma,w}^0 \tau_{\delta,\gamma,w}^9 \quad (4r_D r_T^2 N_v) \quad (1229)$$

Raw expression

$${}^{21}R_{a,\epsilon} \leftarrow - \sum_{\gamma \in A} \sum_{i \in O} \sum_{j \in O} \sum_{k \in O} \sum_{l \in O} \sum_{b \in V} \sum_{c \in V} {}^1T_{c,k} Y_{i,\epsilon}^{2,*} Z_{\epsilon,\gamma}^* Y_{b,\gamma}^{3,*} Y_{j,\gamma}^{4,*} {}^2D_{a,i,b,j} {}^2T_{a,l,b,j} V_{l,i,k,c} \quad (1242)$$

Raw expression

$${}^{21}R_{a,\epsilon} \leftarrow - \sum_{\gamma \in A} \sum_{i \in O} \sum_{j \in O} \sum_{k \in O} \sum_{l \in O} \sum_{b \in V} \sum_{c \in V} {}^1T_{c,k} Y_{i,\epsilon}^{2,*} Z_{\epsilon,\gamma}^* Y_{b,\gamma}^{3,*} Y_{j,\gamma}^{4,*} {}^2D_{a,i,b,j} {}^2T_{a,i,b,l} V_{k,c,l,j} \quad (1230)$$

Factorized expression

$$\tau_{\gamma,\delta,w}^0 = \sum_{i \in O} {}^2D_{i,w}^2 Y_{i,\gamma}^4 Y_{i,\delta}^{2,*} \quad (3r_D r_T^2 N_o) \quad (1243)$$

Factorized expression

$$\tau_{\gamma,\delta,w}^0 = \sum_{i \in O} {}^2D_{i,w}^2 Y_{i,\gamma}^2 Y_{i,\delta}^{2,*} \quad (3r_D r_T^2 N_o) \quad (1231)$$

$$\tau_{\gamma,\delta,w}^1 = \sum_{a \in V} {}^2D_{a,w}^3 Y_{a,\gamma}^1 Y_{a,\delta}^{3,*} \quad (3r_D r_T^2 N_v) \quad (1244)$$

$$\tau_{\gamma,\delta,w}^1 = \sum_{a \in V} {}^2D_{a,w}^3 Y_{a,\gamma}^3 Y_{a,\delta}^{3,*} \quad (3r_D r_T^2 N_v) \quad (1232)$$

$$\tau_{\alpha,i}^2 = \sum_{a \in V} {}^1T_{a,i} W_{a,\alpha}^2 \quad (2r_V N_o N_v) \quad (1245)$$

$$\tau_{\alpha,i}^2 = \sum_{a \in V} {}^1T_{a,i} W_{a,\alpha}^2 \quad (2r_V N_o N_v) \quad (1233)$$

$$\tau_{\alpha}^3 = \sum_{i \in O} W_{i,\alpha}^1 \tau_{\alpha,i}^2 \quad (2r_V N_o) \quad (1246)$$

$$\tau_{\alpha}^3 = \sum_{i \in O} W_{i,\alpha}^1 \tau_{\alpha,i}^2 \quad (2r_V N_o) \quad (1234)$$

$$\tau_{\alpha}^4 = \sum_{\beta \in B} \tau_{\beta}^3 X_{\beta,\alpha} \quad (2r_V^2) \quad (1247)$$

$$\tau_{\alpha}^4 = \sum_{\beta \in B} \tau_{\beta}^3 X_{\beta,\alpha} \quad (2r_V^2) \quad (1235)$$

$$\tau_{i,j}^5 = \sum_{\alpha \in B} \tau_{\alpha}^4 W_{i,\alpha}^3 W_{j,\alpha}^4 \quad (3r_V N_o^2) \quad (1248)$$

$$\tau_{i,j}^5 = \sum_{\alpha \in B} \tau_{\alpha}^4 W_{i,\alpha}^3 W_{j,\alpha}^4 \quad (3r_V N_o^2) \quad (1236)$$

$$\tau_{\gamma,i}^6 = \sum_{j \in O} Y_{j,\gamma}^2 \tau_{j,i}^5 \quad (2r_T N_o^2) \quad (1249)$$

$$\tau_{\gamma,i}^6 = \sum_{j \in O} Y_{j,\gamma}^4 \tau_{j,i}^5 \quad (2r_T N_o^2) \quad (1237)$$

$$\tau_{\gamma,\delta,w}^7 = \sum_{i \in O} {}^2D_{i,w}^4 Y_{i,\delta}^{4,*} \tau_{\gamma,i}^6 \quad (3r_D r_T^2 N_o) \quad (1250)$$

$$\tau_{\gamma,\delta,w}^8 = \sum_{\epsilon \in A} Z_{\delta,\epsilon}^* \tau_{\gamma,\epsilon,w}^1 \tau_{\gamma,\epsilon,w}^7 \quad (3r_D r_T^3) \quad (1251)$$

$$\tau_{\gamma,\delta,w}^9 = \sum_{i \in O} {}^2D_{i,w}^2 Y_{i,\delta}^{2,*} \tau_{\gamma,i}^8 \quad (3r_D r_T^2 N_o) \quad (1264)$$

$$\tau_{\gamma,\delta,w}^9 = \sum_{\epsilon \in A} Z_{\epsilon,\gamma} \tau_{\epsilon,\delta,w}^8 \quad (2r_D r_T^3) \quad (1252)$$

$${}^{21}R_{a,\gamma} \leftarrow - \sum_{\delta \in A} \sum_{w \in D} {}^2D_{a,w}^1 Y_{a,\delta}^1 \tau_{\delta,\gamma,w}^3 \tau_{\delta,\gamma,w}^9 \quad (4r_D r_T^2 N_v) \quad (1265)$$

$${}^{21}R_{a,\gamma} \leftarrow - \sum_{\delta \in A} \sum_{w \in D} {}^2D_{a,w}^1 Y_{a,\delta}^3 \tau_{\delta,\gamma,w}^0 \tau_{\delta,\gamma,w}^9 \quad (4r_D r_T^2 N_v) \quad \text{Raw expression} \quad (1253)$$

$${}^{21}R_{a,\epsilon} \leftarrow - \sum_{\gamma \in A} \sum_{i \in O} \sum_{j \in O} \sum_{k \in O} \sum_{l \in O} \sum_{b \in V} \sum_{c \in V} {}^1T_{c,k} Y_{i,\epsilon}^{2,*} Z_{\epsilon,\gamma}^* Y_{b,\gamma}^{3,*} Y_{j,\gamma}^{4,*} {}^2D_{a,i,b,j} {}^2T_{b,l,a,i} V_{k,c,l,j} \quad (1266)$$

Raw expression

$${}^{21}R_{a,\epsilon} \leftarrow - \sum_{\gamma \in A} \sum_{i \in O} \sum_{j \in O} \sum_{k \in O} \sum_{l \in O} \sum_{b \in V} \sum_{c \in V} {}^1T_{c,k} Y_{i,\epsilon}^{2,*} Z_{\epsilon,\gamma}^* Y_{b,\gamma}^{3,*} Y_{j,\gamma}^{4,*} {}^2D_{a,i,b,j} {}^2T_{b,j,a,l} V_{l,i,k,c} \quad (1254)$$

Factorized expression

$$\tau_{\gamma,\delta,w}^0 = \sum_{a \in V} {}^2D_{a,w}^3 Y_{a,\gamma}^1 Y_{a,\delta}^{3,*} \quad (3r_D r_T^2 N_v) \quad (1267)$$

$$\tau_{\gamma,\delta,w}^0 = \sum_{a \in V} {}^2D_{a,w}^3 Y_{a,\gamma}^3 Y_{a,\delta}^{3,*} \quad (3r_D r_T^2 N_v) \quad (1255)$$

$$\tau_{\gamma,\delta,w}^1 = \sum_{i \in O} {}^2D_{i,w}^4 Y_{i,\gamma}^2 Y_{i,\delta}^{4,*} \quad (3r_D r_T^2 N_o) \quad (1268)$$

$$\tau_{\gamma,\delta,w}^1 = \sum_{i \in O} {}^2D_{i,w}^4 Y_{i,\gamma}^4 Y_{i,\delta}^{4,*} \quad (3r_D r_T^2 N_o) \quad (1256)$$

$$\tau_{\gamma,\delta,w}^2 = \sum_{\epsilon \in A} Z_{\delta,\epsilon}^* \tau_{\gamma,\epsilon,w}^0 \tau_{\gamma,\epsilon,w}^1 \quad (3r_D r_T^3) \quad (1269)$$

$$\tau_{\gamma,\delta,w}^2 = \sum_{\epsilon \in A} Z_{\delta,\epsilon}^* \tau_{\gamma,\epsilon,w}^0 \tau_{\gamma,\epsilon,w}^1 \quad (3r_D r_T^3) \quad (1257)$$

$$\tau_{\gamma,\delta,w}^3 = \sum_{\epsilon \in A} Z_{\epsilon,\gamma} \tau_{\epsilon,\delta,w}^2 \quad (2r_D r_T^3) \quad (1270)$$

$$\tau_{\gamma,\delta,w}^3 = \sum_{\epsilon \in A} Z_{\gamma,\epsilon} \tau_{\epsilon,\delta,w}^2 \quad (2r_D r_T^3) \quad (1258)$$

$$\tau_{\alpha,i}^4 = \sum_{a \in V} {}^1T_{a,i} W_{a,\alpha}^4 \quad (2r_V N_o N_v) \quad (1271)$$

$$\tau_{\alpha,i}^4 = \sum_{a \in V} {}^1T_{a,i} W_{a,\alpha}^4 \quad (2r_V N_o N_v) \quad (1259)$$

$$\tau_{\alpha}^5 = \sum_{i \in O} W_{i,\alpha}^3 \tau_{\alpha,i}^4 \quad (2r_V N_o) \quad (1272)$$

$$\tau_{\alpha}^5 = \sum_{i \in O} W_{i,\alpha}^3 \tau_{\alpha,i}^4 \quad (2r_V N_o) \quad (1260)$$

$$\tau_{\alpha}^6 = \sum_{\beta \in B} \tau_{\beta}^5 X_{\alpha,\beta} \quad (2r_V^2) \quad (1273)$$

$$\tau_{\alpha}^6 = \sum_{\beta \in B} \tau_{\beta}^5 X_{\alpha,\beta} \quad (2r_V^2) \quad (1261)$$

$$\tau_{i,j}^7 = \sum_{\alpha \in B} \tau_{\alpha}^6 W_{i,\alpha}^1 W_{j,\alpha}^2 \quad (3r_V N_o^2) \quad (1274)$$

$$\tau_{i,j}^7 = \sum_{\alpha \in B} \tau_{\alpha}^6 W_{i,\alpha}^1 W_{j,\alpha}^2 \quad (3r_V N_o^2) \quad (1262)$$

$$\tau_{\gamma,i}^8 = \sum_{j \in O} Y_{j,\gamma}^4 \tau_{j,i}^7 \quad (2r_T N_o^2) \quad (1275)$$

$$\tau_{\gamma,i}^8 = \sum_{j \in O} Y_{j,\gamma}^2 \tau_{j,i}^7 \quad (2r_T N_o^2) \quad (1263)$$

$$\tau_{\gamma,\delta,w}^9 = \sum_{i \in O} {}^2D_{i,w}^2 Y_{i,\delta}^{2,*} \tau_{\gamma,i}^8 \quad (3r_D r_T^2 N_o) \quad (1276)$$

$${}^{21}R_{a,\gamma} \leftarrow - \sum_{\delta \in A} \sum_{w \in D} {}^2D^1_{a,w} Y^3_{a,\delta} \tau^3_{\delta,\gamma,w} \tau^9_{\delta,\gamma,w} \quad (4r_D r_T^2 N_v) \quad (1277)$$

Raw expression

$${}^{21}R_{a,\epsilon} \leftarrow \sum_{\gamma \in A} \sum_{i \in O} \sum_{j \in O} \sum_{k \in O} \sum_{b \in V} \sum_{c \in V} \sum_{d \in V} {}^1T_{c,i} Y^{2,*}_{i,\epsilon} Z^*_{\epsilon,\gamma} Y^{3,*}_{b,\gamma} Y^{4,*}_{j,\gamma} {}^2D^{a,i,b,j} {}^2T_{b,j,d,k} V_{a,c,k,d} \quad (1278)$$

Factorized expression

$$\tau^0_{\gamma,\alpha} = \sum_{a \in V} W^2_{a,\alpha} Y^3_{a,\gamma} \quad (2r_T r_V N_v) \quad (1279)$$

$$\tau^1_{\gamma,\alpha,i} = \sum_{\delta \in A} Z_{\gamma,\delta} Y^4_{i,\delta} \tau^0_{\delta,\alpha} \quad (3r_T^2 r_V N_o) \quad (1280)$$

$$\tau^2_{\gamma,\delta,w} = \sum_{a \in V} {}^2D^3_{a,w} Y^1_{a,\gamma} Y^{3,*}_{a,\delta} \quad (3r_D r_T^2 N_v) \quad (1281)$$

$$\tau^3_{\alpha,i,j} = \sum_{\beta \in B} X_{\alpha,\beta} W^3_{i,\beta} W^4_{j,\beta} \quad (3r_V^2 N_o^2) \quad (1282)$$

$$\tau^4_{\gamma,\alpha,i} = \sum_{j \in O} Y^2_{j,\gamma} \tau^3_{\alpha,j,i} \quad (2r_T r_V N_o^2) \quad (1283)$$

$$\tau^5_{\gamma,\delta,\alpha,w} = \sum_{i \in O} {}^2D^4_{i,w} Y^{4,*}_{i,\delta} \tau^2_{\gamma,\delta,w} \tau^4_{\gamma,\alpha,i} \quad (4r_D r_T^2 r_V N_o) \quad (1284)$$

$$\tau^6_{\gamma,\alpha,w,i} = \sum_{\delta \in A} \tau^1_{\delta,\alpha,i} \tau^5_{\delta,\gamma,\alpha,w} \quad (2r_D r_T^2 r_V N_o) \quad (1285)$$

$$\tau^7_{\gamma,w,i,j} = \sum_{\alpha \in B} W^1_{i,\alpha} \tau^6_{\gamma,\alpha,w,j} \quad (2r_D r_T r_V N_o^2) \quad (1286)$$

$$\tau^8_{\gamma,w,i} = \sum_{\delta \in A} \sum_{j \in O} {}^2D^2_{j,w} Y^{2,*}_{j,\gamma} Z^*_{\gamma,\delta} \tau^7_{\delta,w,i,j} \quad (4r_D r_T^2 N_o^2) \quad (1287)$$

$${}^{21}R_{a,\gamma} \leftarrow \sum_{w \in D} \sum_{i \in O} \frac{1}{2} {}^2D^1_{a,w} {}^1T_{a,i} \tau^8_{\gamma,w,i} \quad (3r_D r_T N_o N_v) \quad (1288)$$

Raw expression

$${}^{21}R_{a,\epsilon} \leftarrow \sum_{\gamma \in A} \sum_{i \in O} \sum_{j \in O} \sum_{k \in O} \sum_{b \in V} \sum_{c \in V} \sum_{d \in V} {}^1T_{c,i} Y^{2,*}_{i,\epsilon} Z^*_{\epsilon,\gamma} Y^{3,*}_{b,\gamma} Y^{4,*}_{j,\gamma} {}^2D^{a,i,b,j} {}^2T_{d,k,b,j} V_{a,c,k,d} \quad (1289)$$

Factorized expression

$$\tau^0_{\gamma,\delta,w} = \sum_{a \in V} {}^2D^3_{a,w} Y^3_{a,\gamma} Y^{3,*}_{a,\delta} \quad (3r_D r_T^2 N_v) \quad (1290)$$

$$\tau^1_{\alpha,i,j} = \sum_{\beta \in B} X_{\alpha,\beta} W^3_{i,\beta} W^4_{j,\beta} \quad (3r_V^2 N_o^2) \quad (1291)$$

$$\tau^2_{\gamma,\alpha,i} = \sum_{j \in O} Y^4_{j,\gamma} \tau^1_{\alpha,j,i} \quad (2r_T r_V N_o^2) \quad (1292)$$

$$\tau^3_{\gamma,\delta,\alpha,w} = \sum_{i \in O} {}^2D^4_{i,w} Y^{4,*}_{i,\delta} \tau^0_{\gamma,\delta,w} \tau^2_{\gamma,\alpha,i} \quad (4r_D r_T^2 r_V N_o) \quad (1293)$$

$$\tau^4_{\gamma,\alpha} = \sum_{a \in V} W^2_{a,\alpha} Y^1_{a,\gamma} \quad (2r_T r_V N_v) \quad (1294)$$

$$\tau^5_{\gamma,\alpha,i} = \sum_{\delta \in A} Y^2_{i,\delta} Z_{\delta,\gamma} \tau^4_{\delta,\alpha} \quad (3r_T^2 r_V N_o) \quad (1295)$$

$$\tau^6_{\gamma,\alpha,w,i} = \sum_{\delta \in A} \tau^5_{\delta,\alpha,i} \tau^3_{\delta,\gamma,\alpha,w} \quad (2r_D r_T^2 r_V N_o) \quad (1296)$$

$$\tau^7_{\gamma,w,i,j} = \sum_{\alpha \in B} W^1_{i,\alpha} \tau^6_{\gamma,\alpha,w,j} \quad (2r_D r_T r_V N_o^2) \quad (1297)$$

$$\tau^8_{\gamma,w,i} = \sum_{\delta \in A} \sum_{j \in O} {}^2D^2_{j,w} Y^{2,*}_{j,\gamma} Z^*_{\gamma,\delta} \tau^7_{\delta,w,i,j} \quad (4r_D r_T^2 N_o^2) \quad (1298)$$

$${}^{21}R_{a,\gamma} \leftarrow \sum_{w \in D} \sum_{i \in O} \frac{1}{2} {}^2D^1_{a,w} {}^1T_{a,i} \tau^8_{\gamma,w,i} \quad (3r_D r_T N_o N_v) \quad (1299)$$

Raw expression

$${}^{21}R_{a,\epsilon} \leftarrow \sum_{\gamma \in A} \sum_{i \in O} \sum_{j \in O} \sum_{k \in O} \sum_{b \in V} \sum_{c \in V} \sum_{d \in V} {}^1T_{c,j} Y^{2,*}_{i,\epsilon} Z^*_{\epsilon,\gamma} Y^{3,*}_{b,\gamma} Y^{4,*}_{j,\gamma} {}^2D^{a,i,b,j} {}^2T_{a,i,d,k} V_{b,c,k,d} \quad (1300)$$

Factorized expression

$$\tau^0_{\gamma,\alpha,w} = \sum_{i \in O} {}^2D^2_{i,w} W^2_{i,\alpha} Y^{2,*}_{i,\gamma} \quad (3r_D r_T r_V N_o) \quad (1301)$$

$$\tau^1_{\gamma,\delta,w} = \sum_{a \in V} {}^2D^3_{a,w} Y^1_{a,\gamma} Y^{3,*}_{a,\delta} \quad (3r_D r_T^2 N_v) \quad (1302)$$

$$\tau^2_{\gamma,\alpha} = \sum_{i \in O} W^3_{i,\alpha} Y^2_{i,\gamma} \quad (2r_T r_V N_o) \quad (1303)$$

$$\tau^3_{\gamma,\alpha} = \sum_{a \in V} W^4_{a,\alpha} Y^3_{a,\gamma} \quad (2r_T r_V N_v) \quad (1304)$$

$$\tau^4_{\gamma,\alpha,i} = \sum_{\delta \in A} Z_{\gamma,\delta} Y^4_{i,\delta} \tau^3_{\delta,\alpha} \quad (3r_T^2 r_V N_o) \quad (1305)$$

$$\tau^5_{\gamma,\alpha,w} = \sum_{\delta \in A} \sum_{i \in O} {}^2D^4_{i,w} Y^{4,*}_{i,\gamma} \tau^2_{\delta,\alpha} \tau^1_{\delta,\gamma,w} \tau^4_{\delta,\alpha,i} \quad (5r_D r_T^2 r_V N_o) \quad (1306)$$

$$\tau^6_{\gamma,\alpha,w} = \sum_{\beta \in B} X_{\alpha,\beta} \tau^5_{\gamma,\beta,w} \quad (2r_D r_T r_V^2) \quad (1307)$$

$$\tau^7_{\gamma,\alpha,w} = \sum_{\delta \in A} Z^*_{\gamma,\delta} \tau^6_{\delta,\alpha,w} \quad (2r_D r_T^2 r_V) \quad (1308)$$

$$\tau^8_{\gamma,w,i} = \sum_{\alpha \in B} W^1_{i,\alpha} \tau^0_{\gamma,\alpha,w} \tau^7_{\gamma,\alpha,w} \quad (3r_D r_T r_V N_o) \quad (1309)$$

$${}^{21}R_{a,\gamma} \leftarrow \sum_{w \in D} \sum_{i \in O} \frac{1}{2} {}^2D^1_{a,w} {}^1T_{a,i} \tau^8_{\gamma,w,i} \quad (3r_D r_T N_o N_v) \quad (1310)$$

Raw expression

$${}^{21}R_{a,\epsilon} \leftarrow \sum_{\gamma \in A} \sum_{i \in O} \sum_{j \in O} \sum_{k \in O} \sum_{b \in V} \sum_{c \in V} \sum_{d \in V} {}^1T_{c,j} Y^{2,*}_{i,\epsilon} Z^*_{\epsilon,\gamma} Y^{3,*}_{b,\gamma} Y^{4,*}_{j,\gamma} {}^2D^{a,i,b,j} {}^2T_{d,k,a,i} V_{b,c,k,d} \quad (1311)$$

Factorized expression

$$\tau^0_{\gamma,\alpha,w} = \sum_{i \in O} {}^2D^2_{i,w} W^2_{i,\alpha} Y^{2,*}_{i,\gamma} \quad (3r_D r_T r_V N_o) \quad (1312)$$

$$\tau^1_{\gamma,\delta,w} = \sum_{a \in V} {}^2D^3_{a,w} Y^3_{a,\gamma} Y^{3,*}_{a,\delta} \quad (3r_D r_T^2 N_v) \quad (1313)$$

$$\tau^2_{\gamma,\alpha} = \sum_{a \in V} W^4_{a,\alpha} Y^1_{a,\gamma} \quad (2r_T r_V N_v) \quad (1314)$$

$$\tau^3_{\gamma,\alpha,i} = \sum_{\delta \in A} Y^2_{i,\delta} Z_{\delta,\gamma} \tau^2_{\delta,\alpha} \quad (3r_T^2 r_V N_o) \quad (1315)$$

$$\tau^4_{\gamma,\alpha} = \sum_{i \in O} W^3_{i,\alpha} Y^4_{i,\gamma} \quad (2r_T r_V N_o) \quad (1316)$$

$$\tau^5_{\gamma,\alpha,w} = \sum_{\delta \in A} \sum_{i \in O} {}^2D^4_{i,w} Y^{4,*}_{i,\gamma} \tau^4_{\delta,\alpha} \tau^1_{\delta,\gamma,w} \tau^3_{\delta,\alpha,i} \quad (5r_D r_T^2 r_V N_o) \quad (1317)$$

$$\tau^6_{\gamma,\alpha,w} = \sum_{\beta \in B} X_{\alpha,\beta} \tau^5_{\gamma,\beta,w} \quad (2r_D r_T r_V^2) \quad (1318)$$

$$\tau^7_{\gamma,\alpha,w} = \sum_{\delta \in A} Z^*_{\gamma,\delta} \tau^6_{\delta,\alpha,w} \quad (2r_D r_T^2 r_V) \quad (1319)$$

$$\tau^8_{\gamma,w,i} = \sum_{\alpha \in B} W^1_{i,\alpha} \tau^0_{\gamma,\alpha,w} \tau^7_{\gamma,\alpha,w} \quad (3r_D r_T r_V N_o) \quad (1320)$$

$${}^{21}R_{a,\gamma} \leftarrow \sum_{w \in D} \sum_{i \in O} \frac{1}{2} {}^2D^1_{a,w} {}^1T_{a,i} \tau^8_{\gamma,w,i} \quad (3r_D r_T N_o N_v) \quad (1321)$$

Raw expression

$${}^{21}R_{a,\epsilon} \leftarrow \sum_{\gamma \in A} \sum_{i \in O} \sum_{j \in O} \sum_{k \in O} \sum_{b \in V} \sum_{c \in V} \sum_{d \in V} {}^1T_{c,k} Y^{2,*}_{i,\epsilon} Z^*_{\epsilon,\gamma} Y^{3,*}_{b,\gamma} Y^{4,*}_{j,\gamma} {}^2D^{a,i,b,j} {}^2T_{a,i,d,j} V_{b,d,k,c} \quad (1322)$$

Factorized expression

$$\tau^0_{\alpha,i,j} = \sum_{\beta \in B} W^1_{i,\beta} W^2_{j,\beta} X_{\beta,\alpha} \quad (3r_V^2 N_o^2) \quad (1323)$$

$$\tau^1_{\gamma,\alpha,i} = \sum_{j \in O} Y^4_{j,\gamma} \tau^0_{\alpha,j,i} \quad (2r_T r_V N_o^2) \quad (1324)$$

$$\tau^2_{\gamma,\alpha} = \sum_{a \in V} W^4_{a,\alpha} Y^3_{a,\gamma} \quad (2r_T r_V N_v) \quad (1325)$$

$$\tau^3_{\gamma,i,j} = \sum_{\alpha \in B} W^3_{j,\alpha} \tau^2_{\gamma,\alpha} \tau^1_{\gamma,\alpha,i} \quad (3r_T r_V N_o^2) \quad (1326)$$

$$\tau^4_{\gamma,i,j} = \sum_{\delta \in A} Z_{\gamma,\delta} \tau^3_{\delta,i,j} \quad (2r_T^2 N_o^2) \quad (1327)$$

$$\tau^5_{\gamma,\delta,w} = \sum_{a \in V} {}^2D^3_{a,w} Y^1_{a,\gamma} Y^{3,*}_{a,\delta} \quad (3r_D r_T^2 N_v) \quad (1328)$$

$$\tau^6_{\gamma,\delta,w} = \sum_{i \in O} {}^2D^4_{i,w} Y^2_{i,\gamma} Y^{4,*}_{i,\delta} \quad (3r_D r_T^2 N_o) \quad (1329)$$

$$\tau^7_{\gamma,\delta,w} = \sum_{\epsilon \in A} Z^*_{\delta,\epsilon} \tau^5_{\gamma,\epsilon,w} \tau^6_{\gamma,\epsilon,w} \quad (3r_D r_T^3) \quad (1330)$$

$$\tau^8_{\gamma,w,i,j} = \sum_{\delta \in A} \tau^4_{\delta,i,j} \tau^7_{\delta,\gamma,w} \quad (2r_D r_T^2 N_o^2) \quad (1331)$$

$$\tau^9_{\gamma,w,i} = \sum_{j \in O} {}^2D^2_{j,w} Y^{2,*}_{j,\gamma} \tau^8_{\gamma,w,j,i} \quad (3r_D r_T N_o^2) \quad (1332)$$

$${}^{21}R_{a,\gamma} \leftarrow \sum_{w \in D} \sum_{i \in O} \frac{1}{2} {}^2D^1_{a,w} {}^1T_{a,i} \tau^9_{\gamma,w,i} \quad (3r_D r_T N_o N_v) \quad (1333)$$

Raw expression

$${}^{21}R_{a,\epsilon} \leftarrow \sum_{\gamma \in A} \sum_{i \in O} \sum_{j \in O} \sum_{k \in O} \sum_{b \in V} \sum_{c \in V} \sum_{d \in V} {}^1T_{c,k} Y^{2,*}_{i,\epsilon} Z^*_{\epsilon,\gamma} Y^{3,*}_{b,\gamma} Y^{4,*}_{j,\gamma} {}^2D^{a,i,b,j} {}^2T_{b,j,d,i} V_{a,d,k,c} \quad (1334)$$

Factorized expression

$$\tau^0_{\alpha,i,j} = \sum_{\beta \in B} W^1_{i,\beta} W^2_{j,\beta} X_{\beta,\alpha} \quad (3r_V^2 N_o^2) \quad (1335)$$

$$\tau^1_{\gamma,\alpha,i} = \sum_{j \in O} Y^2_{j,\gamma} \tau^0_{\alpha,j,i} \quad (2r_T r_V N_o^2) \quad (1336)$$

$$\tau^2_{\gamma,\alpha} = \sum_{a \in V} W^4_{a,\alpha} Y^1_{a,\gamma} \quad (2r_T r_V N_v) \quad (1337)$$

$$\tau^3_{\gamma,i,j} = \sum_{\alpha \in B} W^3_{j,\alpha} \tau^2_{\gamma,\alpha} \tau^1_{\gamma,\alpha,i} \quad (3r_T r_V N_o^2) \quad (1338)$$

$$\tau^4_{\gamma,i,j} = \sum_{\delta \in A} Z_{\delta,\gamma} \tau^3_{\delta,i,j} \quad (2r_T^2 N_o^2) \quad (1339)$$

$$\tau^5_{\gamma,\delta,w} = \sum_{a \in V} {}^2D^3_{a,w} Y^3_{a,\gamma} Y^{3,*}_{a,\delta} \quad (3r_D r_T^2 N_v) \quad (1340)$$

$$\tau^6_{\gamma,\delta,w} = \sum_{i \in O} {}^2D^4_{i,w} Y^4_{i,\gamma} Y^{4,*}_{i,\delta} \quad (3r_D r_T^2 N_o) \quad (1341)$$

$$\tau^7_{\gamma,\delta,w} = \sum_{\epsilon \in A} Z^*_{\delta,\epsilon} \tau^5_{\gamma,\epsilon,w} \tau^6_{\gamma,\epsilon,w} \quad (3r_D r_T^3) \quad (1342)$$

$$\tau^8_{\gamma,w,i,j} = \sum_{\delta \in A} \tau^4_{\delta,i,j} \tau^7_{\delta,\gamma,w} \quad (2r_D r_T^2 N_o^2) \quad (1343)$$

$$\tau^9_{\gamma,w,i} = \sum_{j \in O} {}^2D^2_{j,w} Y^{2,*}_{j,\gamma} \tau^8_{\gamma,w,j,i} \quad (3r_D r_T N_o^2) \quad (1344)$$

$${}^{21}R_{a,\gamma} \leftarrow \sum_{w \in D} \sum_{i \in O} \frac{1}{2} {}^2D^1_{a,w} {}^1T_{a,i} \tau^9_{\gamma,w,i} \quad (3r_D r_T N_o N_v) \quad (1345)$$

Raw expression

$${}^{21}R_{a,\epsilon} \leftarrow \sum_{\gamma \in A} \sum_{i \in O} \sum_{j \in O} \sum_{k \in O} \sum_{b \in V} \sum_{c \in V} \sum_{d \in V} {}^1T_{c,k} Y^{2,*}_{i,\epsilon} Z^*_{\epsilon,\gamma} Y^{3,*}_{b,\gamma} Y^{4,*}_{j,\gamma} {}^2D^{a,i,b,j} {}^2T_{d,i,b,j} V_{a,d,k,c} \quad (1346)$$

Factorized expression

$$\tau^0_{\gamma,\delta,w} = \sum_{i \in O} {}^2D^2_{i,w} Y^2_{i,\gamma} Y^{2,*}_{i,\delta} \quad (3r_D r_T^2 N_o) \quad (1347)$$

$$\tau^1_{\gamma,w,i} = \sum_{a \in V} {}^2D^3_{a,w} {}^1T_{a,i} Y^{3,*}_{a,\gamma} \quad (3r_D r_T N_o N_v) \quad (1348)$$

$$\tau^2_{\gamma,\alpha} = \sum_{a \in V} W^2_{a,\alpha} Y^3_{a,\gamma} \quad (2r_T r_V N_v) \quad (1349)$$

$$\tau^3_{\alpha,i,j} = \sum_{\beta \in B} X_{\alpha,\beta} W^3_{i,\beta} W^4_{j,\beta} \quad (3r_V^2 N_o^2) \quad (1350)$$

$$\tau^4_{\gamma,\alpha,i} = \sum_{j \in O} Y^4_{j,\gamma} \tau^3_{\alpha,j,i} \quad (2r_T r_V N_o^2) \quad (1351)$$

$$\tau^5_{\gamma,i,j} = \sum_{\alpha \in B} W^1_{i,\alpha} \tau^2_{\gamma,\alpha} \tau^4_{\gamma,\alpha,j} \quad (3r_T r_V N_o^2) \quad (1352)$$

$$\tau^6_{\gamma,i,j} = \sum_{\delta \in A} Z_{\gamma,\delta} \tau^5_{\delta,i,j} \quad (2r_T^2 N_o^2) \quad (1353)$$

$$\tau^7_{\gamma,\delta,w} = \sum_{i \in O} \sum_{j \in O} {}^2D^4_{i,w} Y^{4,*}_{i,\delta} \tau^1_{\delta,w,j} \tau^6_{\gamma,j,i} \quad (4r_D r_T^2 N_o^2) \quad (1354)$$

$$\tau^8_{\gamma,\delta,w} = \sum_{\epsilon \in A} Z^*_{\delta,\epsilon} \tau^7_{\gamma,\epsilon,w} \quad (2r_D r_T^3) \quad (1355)$$

$${}^{21}R_{a,\gamma} \leftarrow \sum_{\delta \in A} \sum_{w \in D} \frac{1}{2} {}^2D^1_{a,w} Y^1_{a,\delta} \tau^0_{\delta,\gamma,w} \tau^8_{\delta,\gamma,w} \quad (4r_D r_T^2 N_v) \quad (1356)$$

Raw expression

$${}^{21}R_{a,\epsilon} \leftarrow \sum_{\gamma \in A} \sum_{i \in O} \sum_{j \in O} \sum_{k \in O} \sum_{b \in V} \sum_{c \in V} \sum_{d \in V} {}^1T_{c,k} Y^{2,*}_{i,\epsilon} Z^*_{\epsilon,\gamma} Y^{3,*}_{b,\gamma} Y^{4,*}_{j,\gamma} {}^2D^{a,i,b,j} {}^2T_{d,j,a,i} V_{b,d,k,c} \quad (1357)$$

Factorized expression

$$\tau^0_{\gamma,\delta,w} = \sum_{i \in O} {}^2D^2_{i,w} Y^4_{i,\gamma} Y^{2,*}_{i,\delta} \quad (3r_D r_T^2 N_o) \quad (1358)$$

$$\tau^1_{\gamma,w,i} = \sum_{a \in V} {}^2D^3_{a,w} {}^1T_{a,i} Y^{3,*}_{a,\gamma} \quad (3r_D r_T N_o N_v) \quad (1359)$$

$$\tau^2_{\gamma,\alpha} = \sum_{a \in V} W^2_{a,\alpha} Y^1_{a,\gamma} \quad (2r_T r_V N_v) \quad (1360)$$

$$\tau^3_{\alpha,i,j} = \sum_{\beta \in B} X_{\alpha,\beta} W^3_{i,\beta} W^4_{j,\beta} \quad (3r_V^2 N_o^2) \quad (1361)$$

$$\tau^4_{\gamma,\alpha,i} = \sum_{j \in O} Y^2_{j,\gamma} \tau^3_{\alpha,j,i} \quad (2r_T r_V N_o^2) \quad (1362)$$

$$\tau^5_{\gamma,i,j} = \sum_{\alpha \in B} W^1_{i,\alpha} \tau^2_{\gamma,\alpha} \tau^4_{\gamma,\alpha,j} \quad (3r_T r_V N_o^2) \quad (1363)$$

$$\tau^6_{\gamma,i,j} = \sum_{\delta \in A} Z_{\delta,\gamma} \tau^5_{\delta,i,j} \quad (2r_T^2 N_o^2) \quad (1364)$$

$$\tau^7_{\gamma,\delta,w} = \sum_{i \in O} \sum_{j \in O} {}^2D^4_{i,w} Y^{4,*}_{i,\delta} \tau^1_{\delta,w,j} \tau^6_{\gamma,j,i} \quad (4r_D r_T^2 N_o^2) \quad (1365)$$

$$\tau^8_{\gamma,\delta,w} = \sum_{\epsilon \in A} Z^*_{\delta,\epsilon} \tau^7_{\gamma,\epsilon,w} \quad (2r_D r_T^3) \quad (1366)$$

$${}^{21}R_{a,\gamma} \leftarrow \sum_{\delta \in A} \sum_{w \in D} \frac{1}{2} {}^2D^1_{a,w} Y^3_{a,\delta} \tau^0_{\delta,\gamma,w} \tau^8_{\delta,\gamma,w} \quad (4r_D r_T^2 N_v) \quad (1367)$$

Raw expression

$${}^{21}R_{a,\epsilon} \leftarrow - \sum_{\gamma \in A} \sum_{i \in O} \sum_{j \in O} \sum_{k \in O} \sum_{b \in V} \sum_{c \in V} \sum_{d \in V} \frac{1}{2} {}^1T_{a,k} Y^{2,*}_{i,\epsilon} Z^*_{\epsilon,\gamma} Y^{3,*}_{b,\gamma} Y^{4,*}_{j,\gamma} {}^2D^{a,i,b,j} {}^2T_{c,i,d,j} V_{b,d,k,c} \quad (1368)$$

Factorized expression

$$\tau^0_{\gamma,\alpha} = \sum_{i \in O} W^1_{i,\alpha} Y^2_{i,\gamma} \quad (2r_T r_V N_o) \quad (1369)$$

$$\tau^1_{\gamma,\alpha} = \sum_{a \in V} W^2_{a,\alpha} Y^3_{a,\gamma} \quad (2r_T r_V N_v) \quad (1370)$$

$$\tau^2_{\gamma,\alpha,i} = \sum_{\delta \in A} Z_{\gamma,\delta} Y^4_{i,\delta} \tau^1_{\delta,\alpha} \quad (3r_T^2 r_V N_o) \quad (1371)$$

$$\tau^3_{\gamma,w,i} = \sum_{a \in V} {}^2D^3_{a,w} {}^1T_{a,i} Y^{3,*}_{a,\gamma} \quad (3r_D r_T N_o N_v) \quad (1372)$$

$$\tau^4_{\gamma,\alpha,w} = \sum_{i \in O} W^3_{i,\alpha} \tau^3_{\gamma,w,i} \quad (2r_D r_T r_V N_o) \quad (1373)$$

$$\tau^5_{\gamma,\alpha,w} = \sum_{i \in O} {}^2D^4_{i,w} W^4_{i,\alpha} Y^{4,*}_{i,\gamma} \quad (3r_D r_T r_V N_o) \quad (1374)$$

$$\tau^6_{\gamma,\alpha,w} = \sum_{\beta \in B} X_{\alpha,\beta} \tau^4_{\gamma,\beta,w} \tau^5_{\gamma,\beta,w} \quad (3r_D r_T r_V^2) \quad (1375)$$

$$\tau^7_{\gamma,\alpha,w} = \sum_{\delta \in A} Z^*_{\gamma,\delta} \tau^6_{\delta,\alpha,w} \quad (2r_D r_T^2 r_V) \quad (1376)$$

$$\tau_{\gamma,\delta,w,i}^8 = \sum_{\alpha \in B} \tau_{\gamma,\alpha}^0 \tau_{\gamma,\alpha,i}^2 \tau_{\delta,\alpha,w}^7 \quad (3r_D r_T^2 r_V N_o) \quad (1377)$$

$$\tau_{\gamma,\delta,w,i}^8 = \sum_{\alpha \in B} \tau_{\gamma,\alpha}^2 \tau_{\gamma,\alpha,i}^1 \tau_{\delta,\alpha,w}^7 \quad (3r_D r_T^2 r_V N_o) \quad (1389)$$

$$\tau_{\gamma,\delta,w}^9 = \sum_{i \in O} {}^2D_{i,w}^2 Y_{i,\delta}^{2,*} \tau_{\gamma,\delta,w,i}^8 \quad (3r_D r_T^2 N_o) \quad (1378)$$

$$\tau_{\gamma,\delta,w}^9 = \sum_{i \in O} {}^2D_{i,w}^2 Y_{i,\delta}^{2,*} \tau_{\gamma,\delta,w,i}^8 \quad (3r_D r_T^2 N_o) \quad (1390)$$

$${}^{21}R_{a,\gamma} \leftarrow \sum_{\delta \in A} \sum_{w \in D} \frac{1}{2} {}^2D_{a,w}^1 Y_{a,\delta}^1 \tau_{\delta,\gamma,w}^9 \quad (3r_D r_T^2 N_v) \quad (1379)$$

$${}^{21}R_{a,\gamma} \leftarrow \sum_{\delta \in A} \sum_{w \in D} \frac{1}{2} {}^2D_{a,w}^1 Y_{a,\delta}^3 \tau_{\delta,\gamma,w}^9 \quad (3r_D r_T^2 N_v) \quad (1391)$$

Raw expression

$${}^{21}R_{a,\epsilon} \leftarrow - \sum_{\gamma \in A} \sum_{i \in O} \sum_{j \in O} \sum_{k \in O} \sum_{b \in V} \sum_{c \in V} \sum_{d \in V} \frac{1}{2} {}^1T_{a,k} Y_{i,\epsilon}^{2,*} Z_{\epsilon,\gamma}^* Y_{b,\gamma}^{3,*} Y_{j,\gamma}^{4,*} {}^2D_{a,i,b,j} {}^2T_{c,j,d,i} V_{b,c,k,d} \quad (1380)$$

Raw expression

$${}^{21}R_{a,\epsilon} \leftarrow - \sum_{\gamma \in A} \sum_{i \in O} \sum_{j \in O} \sum_{k \in O} \sum_{b \in V} \sum_{c \in V} \sum_{d \in V} \frac{1}{2} {}^1T_{b,k} Y_{i,\epsilon}^{2,*} Z_{\epsilon,\gamma}^* Y_{b,\gamma}^{3,*} Y_{j,\gamma}^{4,*} {}^2D_{a,i,b,j} {}^2T_{c,i,d,j} V_{a,c,k,d} \quad (1392)$$

Factorized expression

$$\tau_{\gamma,\alpha}^0 = \sum_{a \in V} W_{a,\alpha}^2 Y_{a,\gamma}^1 \quad (2r_T r_V N_v) \quad (1381)$$

$$\tau_{\alpha,i,j}^0 = \sum_{\beta \in B} W_{i,\beta}^1 W_{j,\beta}^2 X_{\beta,\alpha} \quad (3r_V^2 N_o^2) \quad (1393)$$

$$\tau_{\gamma,\alpha,i}^1 = \sum_{\delta \in A} Y_{i,\delta}^2 Z_{\delta,\gamma} \tau_{\delta,\alpha}^0 \quad (3r_T^2 r_V N_o) \quad (1382)$$

$$\tau_{\gamma,\alpha,i}^1 = \sum_{j \in O} Y_{j,\gamma}^2 \tau_{\alpha,j,i}^0 \quad (2r_T r_V N_o^2) \quad (1394)$$

$$\tau_{\gamma,\alpha}^2 = \sum_{i \in O} W_{i,\alpha}^1 Y_{i,\gamma}^4 \quad (2r_T r_V N_o) \quad (1383)$$

$$\tau_{\gamma,w,i}^2 = \sum_{a \in V} {}^2D_{a,w}^3 {}^1T_{a,i} Y_{a,\gamma}^{3,*} \quad (3r_D r_T N_o N_v) \quad (1395)$$

$$\tau_{\gamma,w,i}^3 = \sum_{a \in V} {}^2D_{a,w}^3 {}^1T_{a,i} Y_{a,\gamma}^{3,*} \quad (3r_D r_T N_o N_v) \quad (1384)$$

$$\tau_{\gamma,w,i,j}^3 = \sum_{\delta \in A} {}^2D_{i,w}^4 Z_{\gamma,\delta}^* Y_{i,\delta}^{4,*} \tau_{\delta,w,j}^2 \quad (4r_D r_T^2 N_o^2) \quad (1396)$$

$$\tau_{\gamma,\alpha,w}^4 = \sum_{i \in O} W_{i,\alpha}^3 \tau_{\gamma,w,i}^3 \quad (2r_D r_T r_V N_o) \quad (1385)$$

$$\tau_{\gamma,\alpha,w,i}^4 = \sum_{j \in O} W_{j,\alpha}^3 \tau_{\gamma,w,i,j}^3 \quad (2r_D r_T r_V N_o^2) \quad (1397)$$

$$\tau_{\gamma,\alpha,w}^5 = \sum_{i \in O} {}^2D_{i,w}^4 W_{i,\alpha}^4 Y_{i,\gamma}^{4,*} \quad (3r_D r_T r_V N_o) \quad (1386)$$

$$\tau_{\gamma,\alpha}^5 = \sum_{a \in V} W_{a,\alpha}^4 Y_{a,\gamma}^3 \quad (2r_T r_V N_v) \quad (1398)$$

$$\tau_{\gamma,\alpha,w}^6 = \sum_{\beta \in B} X_{\alpha,\beta} \tau_{\gamma,\beta,w}^4 \tau_{\gamma,\beta,w}^5 \quad (3r_D r_T r_V^2) \quad (1387)$$

$$\tau_{\gamma,\alpha,i}^6 = \sum_{\delta \in A} Z_{\gamma,\delta} Y_{i,\delta}^4 \tau_{\delta,\alpha}^5 \quad (3r_T^2 r_V N_o) \quad (1399)$$

$$\tau_{\gamma,\alpha,w}^7 = \sum_{\delta \in A} Z_{\gamma,\delta}^* \tau_{\delta,\alpha,w}^6 \quad (2r_D r_T^2 r_V) \quad (1388)$$

$$\tau_{\gamma,\delta,\alpha,w}^7 = \sum_{i \in O} \tau_{\gamma,\alpha,i}^6 \tau_{\delta,\alpha,w,i}^4 \quad (2r_D r_T^2 r_V N_o) \quad (1400)$$



$$\tau^8_{\gamma,\delta,w,i} = \sum_{\alpha \in B} \tau^1_{\gamma,\alpha,i} \tau^7_{\gamma,\delta,\alpha,w} \quad (2r_D r_T^2 r_V N_o) \quad (1401)$$

$$\tau^8_{\gamma,\delta,w,i} = \sum_{\alpha \in B} \tau^1_{\gamma,\alpha,i} \tau^7_{\gamma,\delta,\alpha,w} \quad (2r_D r_T^2 r_V N_o) \quad (1413)$$

$$\tau^9_{\gamma,\delta,w} = \sum_{i \in O} {}^2D^2_{i,w} Y^{2,*}_{i,\delta} \tau^8_{\gamma,\delta,w,i} \quad (3r_D r_T^2 N_o) \quad (1402)$$

$$\tau^9_{\gamma,\delta,w} = \sum_{i \in O} {}^2D^2_{i,w} Y^{2,*}_{i,\delta} \tau^8_{\gamma,\delta,w,i} \quad (3r_D r_T^2 N_o) \quad (1414)$$

$${}^{21}R_{a,\gamma} \leftarrow \sum_{\delta \in A} \sum_{w \in D} \frac{1}{2} {}^2D^1_{a,w} Y^1_{a,\delta} \tau^9_{\delta,\gamma,w} \quad (3r_D r_T^2 N_v) \quad (1403)$$

$${}^{21}R_{a,\gamma} \leftarrow \sum_{\delta \in A} \sum_{w \in D} \frac{1}{2} {}^2D^1_{a,w} Y^3_{a,\delta} \tau^9_{\delta,\gamma,w} \quad (3r_D r_T^2 N_v) \quad (1415)$$

Raw expression

$${}^{21}R_{a,\epsilon} \leftarrow - \sum_{\gamma \in A} \sum_{i \in O} \sum_{j \in O} \sum_{k \in O} \sum_{b \in V} \sum_{c \in V} \sum_{d \in V} \frac{1}{2} {}^1T_{b,k} Y^{2,*}_{i,\epsilon} Z^*_{\epsilon,\gamma} Y^{3,*}_{b,\gamma} Y^{4,*}_{j,\gamma} {}^2D^{a,i,b,j} {}^2T_{c,j,d,i} V_{a,d,k,c} \quad (1404)$$

Raw expression

$${}^{21}R_{a,\epsilon} \leftarrow - \sum_{\gamma \in A} \sum_{i \in O} \sum_{j \in O} \sum_{k \in O} \sum_{b \in V} \sum_{c \in V} \sum_{d \in V} \frac{1}{2} {}^1T_{c,i} Y^{2,*}_{i,\epsilon} Z^*_{\epsilon,\gamma} Y^{3,*}_{b,\gamma} Y^{4,*}_{j,\gamma} {}^2D^{a,i,b,j} {}^2T_{a,k,d,j} V_{b,d,k,c} \quad (1416)$$

Factorized expression

$$\tau^0_{\alpha,i,j} = \sum_{\beta \in B} W^1_{i,\beta} W^2_{j,\beta} X_{\beta,\alpha} \quad (3r_V^2 N_o^2) \quad (1405)$$

$$\tau^0_{\gamma,\alpha,w} = \sum_{i \in O} {}^2D^4_{i,w} W^4_{i,\alpha} Y^{4,*}_{i,\gamma} \quad (3r_D r_T r_V N_o) \quad (1417)$$

$$\tau^1_{\gamma,\alpha,i} = \sum_{j \in O} Y^4_{j,\gamma} \tau^0_{\alpha,j,i} \quad (2r_T r_V N_o^2) \quad (1406)$$

$$\tau^1_{\gamma,\delta,w} = \sum_{a \in V} {}^2D^3_{a,w} Y^3_{a,\gamma} Y^{3,*}_{a,\delta} \quad (3r_D r_T^2 N_v) \quad (1418)$$

$$\tau^2_{\gamma,w,i} = \sum_{a \in V} {}^2D^3_{a,w} {}^1T_{a,i} Y^{3,*}_{a,\gamma} \quad (3r_D r_T N_o N_v) \quad (1407)$$

$$\tau^2_{\gamma,\delta,w,i} = \sum_{\epsilon \in A} Z_{\gamma,\epsilon} Y^4_{i,\epsilon} \tau^1_{\epsilon,\delta,w} \quad (3r_D r_T^3 N_o) \quad (1419)$$

$$\tau^3_{\gamma,w,i,j} = \sum_{\delta \in A} {}^2D^4_{i,w} Z^*_{\gamma,\delta} Y^{4,*}_{i,\delta} \tau^2_{\delta,w,j} \quad (4r_D r_T^2 N_o^2) \quad (1408)$$

$$\tau^3_{\gamma,\delta,\alpha,w} = \sum_{i \in O} W^3_{i,\alpha} \tau^0_{\delta,\alpha,w} \tau^2_{\gamma,\delta,w,i} \quad (3r_D r_T^2 r_V N_o) \quad (1420)$$

$$\tau^4_{\gamma,\alpha,w,i} = \sum_{j \in O} W^3_{j,\alpha} \tau^3_{\gamma,w,i,j} \quad (2r_D r_T r_V N_o^2) \quad (1409)$$

$$\tau^4_{\alpha,i} = \sum_{a \in V} {}^1T_{a,i} W^2_{a,\alpha} \quad (2r_V N_o N_v) \quad (1421)$$

$$\tau^5_{\gamma,\alpha} = \sum_{a \in V} W^4_{a,\alpha} Y^1_{a,\gamma} \quad (2r_T r_V N_v) \quad (1410)$$

$$\tau^5_{\alpha,i,j} = \sum_{\beta \in B} W^1_{j,\beta} X_{\beta,\alpha} \tau^4_{\beta,i} \quad (3r_V^2 N_o^2) \quad (1422)$$

$$\tau^6_{\gamma,\alpha,i} = \sum_{\delta \in A} Y^2_{i,\delta} Z_{\delta,\gamma} \tau^5_{\delta,\alpha} \quad (3r_T^2 r_V N_o) \quad (1411)$$

$$\tau^6_{\gamma,\alpha,i} = \sum_{j \in O} Y^2_{j,\gamma} \tau^5_{\alpha,i,j} \quad (2r_T r_V N_o^2) \quad (1423)$$

$$\tau^7_{\gamma,\delta,\alpha,w} = \sum_{i \in O} \tau^6_{\gamma,\alpha,i} \tau^4_{\delta,\alpha,w,i} \quad (2r_D r_T^2 r_V N_o) \quad (1412)$$

$$\tau^7_{\gamma,\delta,w,i} = \sum_{\alpha \in B} \tau^6_{\gamma,\alpha,i} \tau^3_{\gamma,\delta,\alpha,w} \quad (2r_D r_T^2 r_V N_o) \quad (1424)$$

$$\tau_{\gamma,\delta,w}^8 = \sum_{\epsilon \in A} \sum_{i \in O} {}^2D_{i,w}^2 Y_{i,\delta}^{2,*} Z_{\delta,\epsilon}^* \tau_{\gamma,\epsilon,w,i}^7 \quad (4r_D r_T^3 N_o) \quad (1425)$$

$${}^{21}R_{a,\gamma} \leftarrow \sum_{\delta \in A} \sum_{w \in D} \frac{1}{2} {}^2D_{a,w}^1 Y_{a,\delta}^1 \tau_{\delta,\gamma,w}^8 \quad (3r_D r_T^2 N_v) \quad (1426)$$

Raw expression

$${}^{21}R_{a,\epsilon} \leftarrow - \sum_{\gamma \in A} \sum_{i \in O} \sum_{j \in O} \sum_{k \in O} \sum_{b \in V} \sum_{c \in V} \sum_{d \in V} \frac{1}{2} {}^1T_{c,i} Y_{i,\epsilon}^{2,*} Z_{\epsilon,\gamma}^* Y_{b,\gamma}^{3,*} Y_{j,\gamma}^{4,*} {}^2D_{a,i,b,j} {}^2T_{b,j,d,k} V_{a,d,k,c} \quad (1427)$$

Factorized expression

$$\tau_{\gamma,\alpha,w}^0 = \sum_{i \in O} {}^2D_{i,w}^4 W_{i,\alpha}^4 Y_{i,\gamma}^{4,*} \quad (3r_D r_T r_V N_o) \quad (1428)$$

$$\tau_{\gamma,\delta,w}^1 = \sum_{a \in V} {}^2D_{a,w}^3 Y_{a,\gamma}^1 Y_{a,\delta}^{3,*} \quad (3r_D r_T^2 N_v) \quad (1429)$$

$$\tau_{\gamma,\delta,w,i}^2 = \sum_{\epsilon \in A} Y_{i,\epsilon}^2 Z_{\epsilon,\gamma} \tau_{\epsilon,\delta,w}^1 \quad (3r_D r_T^3 N_o) \quad (1430)$$

$$\tau_{\gamma,\delta,\alpha,w}^3 = \sum_{i \in O} W_{i,\alpha}^3 \tau_{\delta,\alpha,w}^0 \tau_{\gamma,\delta,w,i}^2 \quad (3r_D r_T^2 r_V N_o) \quad (1431)$$

$$\tau_{\alpha,i}^4 = \sum_{a \in V} {}^1T_{a,i} W_{a,\alpha}^2 \quad (2r_V N_o N_v) \quad (1432)$$

$$\tau_{\alpha,i,j}^5 = \sum_{\beta \in B} W_{j,\beta}^1 X_{\beta,\alpha} \tau_{\beta,i}^4 \quad (3r_V^2 N_o^2) \quad (1433)$$

$$\tau_{\gamma,\alpha,i}^6 = \sum_{j \in O} Y_{j,\gamma}^4 \tau_{\alpha,i,j}^5 \quad (2r_T r_V N_o^2) \quad (1434)$$

$$\tau_{\gamma,\delta,w,i}^7 = \sum_{\alpha \in B} \tau_{\gamma,\alpha,i}^6 \tau_{\gamma,\delta,\alpha,w}^3 \quad (2r_D r_T^2 r_V N_o) \quad (1435)$$

$$\tau_{\gamma,\delta,w}^8 = \sum_{\epsilon \in A} \sum_{i \in O} {}^2D_{i,w}^2 Y_{i,\delta}^{2,*} Z_{\delta,\epsilon}^* \tau_{\gamma,\epsilon,w,i}^7 \quad (4r_D r_T^3 N_o) \quad (1436)$$

$${}^{21}R_{a,\gamma} \leftarrow \sum_{\delta \in A} \sum_{w \in D} \frac{1}{2} {}^2D_{a,w}^1 Y_{a,\delta}^3 \tau_{\delta,\gamma,w}^8 \quad (3r_D r_T^2 N_v) \quad (1437)$$

Raw expression

$${}^{21}R_{a,\epsilon} \leftarrow - \sum_{\gamma \in A} \sum_{i \in O} \sum_{j \in O} \sum_{k \in O} \sum_{b \in V} \sum_{c \in V} \sum_{d \in V} \frac{1}{2} {}^1T_{c,i} Y_{i,\epsilon}^{2,*} Z_{\epsilon,\gamma}^* Y_{b,\gamma}^{3,*} Y_{j,\gamma}^{4,*} {}^2D_{a,i,b,j} {}^2T_{b,k,d,j} V_{a,c,k,d} \quad (1438)$$

Factorized expression

$$\tau_{\alpha,i}^0 = \sum_{a \in V} {}^1T_{a,i} W_{a,\alpha}^4 \quad (2r_V N_o N_v) \quad (1439)$$

$$\tau_{\gamma,\alpha,w}^1 = \sum_{i \in O} {}^2D_{i,w}^4 Y_{i,\gamma}^{4,*} \tau_{\alpha,i}^0 \quad (3r_D r_T r_V N_o) \quad (1440)$$

$$\tau_{\gamma,\delta,w}^2 = \sum_{a \in V} {}^2D_{a,w}^3 Y_{a,\gamma}^3 Y_{a,\delta}^{3,*} \quad (3r_D r_T^2 N_v) \quad (1441)$$

$$\tau_{\gamma,\delta,w,i}^3 = \sum_{\epsilon \in A} Z_{\gamma,\epsilon} Y_{i,\epsilon}^4 \tau_{\epsilon,\delta,w}^2 \quad (3r_D r_T^3 N_o) \quad (1442)$$

$$\tau_{\gamma,\delta,\alpha,w}^4 = \sum_{i \in O} W_{i,\alpha}^3 \tau_{\delta,\alpha,w}^1 \tau_{\gamma,\delta,w,i}^3 \quad (3r_D r_T^2 r_V N_o) \quad (1443)$$

$$\tau_{\alpha,i,j}^5 = \sum_{\beta \in B} W_{i,\beta}^1 W_{j,\beta}^2 X_{\beta,\alpha} \quad (3r_V^2 N_o^2) \quad (1444)$$

$$\tau_{\gamma,\alpha,i}^6 = \sum_{j \in O} Y_{j,\gamma}^2 \tau_{\alpha,j,i}^5 \quad (2r_T r_V N_o^2) \quad (1445)$$

$$\tau_{\gamma,\delta,w,i}^7 = \sum_{\alpha \in B} \tau_{\gamma,\alpha,i}^6 \tau_{\gamma,\delta,\alpha,w}^4 \quad (2r_D r_T^2 r_V N_o) \quad (1446)$$

$$\tau_{\gamma,\delta,w}^8 = \sum_{\epsilon \in A} \sum_{i \in O} {}^2D_{i,w}^2 Y_{i,\delta}^{2,*} Z_{\delta,\epsilon}^* \tau_{\gamma,\epsilon,w,i}^7 \quad (4r_D r_T^3 N_o) \quad (1447)$$

$${}^{21}R_{a,\gamma} \leftarrow \sum_{\delta \in A} \sum_{w \in D} \frac{1}{2} {}^2D_{a,w}^1 Y_{a,\delta}^1 \tau_{\delta,\gamma,w}^8 \quad (3r_D r_T^2 N_v) \quad (1448)$$

Raw expression

$${}^{21}R_{a,\epsilon} \leftarrow - \sum_{\gamma \in A} \sum_{i \in O} \sum_{j \in O} \sum_{k \in O} \sum_{b \in V} \sum_{c \in V} \sum_{d \in V} \frac{1}{2} {}^1T_{c,i} Y^{2,*}_{i,\epsilon} Z^*_{\epsilon,\gamma} Y^{3,*}_{b,\gamma} Y^{4,*}_{j,\gamma} {}^2D^{a,i,b,j} {}^2T_{d,j,a,k} V_{b,d,k,c} \quad (1449)$$

Factorized expression

$$\tau^0_{\alpha,i} = \sum_{a \in V} {}^1T_{a,i} W^4_{a,\alpha} \quad (2r_V N_o N_v) \quad (1450)$$

$$\tau^1_{\gamma,\alpha,w} = \sum_{i \in O} {}^2D^4_{i,w} Y^{4,*}_{i,\gamma} \tau^0_{\alpha,i} \quad (3r_D r_T r_V N_o) \quad (1451)$$

$$\tau^2_{\gamma,\delta,w} = \sum_{a \in V} {}^2D^3_{a,w} Y^1_{a,\gamma} Y^{3,*}_{a,\delta} \quad (3r_D r_T^2 N_v) \quad (1452)$$

$$\tau^3_{\gamma,\delta,w,i} = \sum_{\epsilon \in A} Y^2_{i,\epsilon} Z_{\epsilon,\gamma} \tau^2_{\epsilon,\delta,w} \quad (3r_D r_T^3 N_o) \quad (1453)$$

$$\tau^4_{\gamma,\delta,\alpha,w} = \sum_{i \in O} W^3_{i,\alpha} \tau^1_{\delta,\alpha,w} \tau^3_{\gamma,\delta,w,i} \quad (3r_D r_T^2 r_V N_o) \quad (1454)$$

$$\tau^5_{\alpha,i,j} = \sum_{\beta \in B} W^1_{i,\beta} W^2_{j,\beta} X_{\beta,\alpha} \quad (3r_V^2 N_o^2) \quad (1455)$$

$$\tau^6_{\gamma,\alpha,i} = \sum_{j \in O} Y^4_{j,\gamma} \tau^5_{\alpha,j,i} \quad (2r_T r_V N_o^2) \quad (1456)$$

$$\tau^7_{\gamma,\delta,w,i} = \sum_{\alpha \in B} \tau^6_{\gamma,\alpha,i} \tau^4_{\gamma,\delta,\alpha,w} \quad (2r_D r_T^2 r_V N_o) \quad (1457)$$

$$\tau^8_{\gamma,\delta,w} = \sum_{\epsilon \in A} \sum_{i \in O} {}^2D^2_{i,w} Y^{2,*}_{i,\delta} Z^*_{\delta,\epsilon} \tau^7_{\gamma,\epsilon,w,i} \quad (4r_D r_T^3 N_o) \quad (1458)$$

$${}^{21}R_{a,\gamma} \leftarrow \sum_{\delta \in A} \sum_{w \in D} \frac{1}{2} {}^2D^1_{a,w} Y^3_{a,\delta} \tau^8_{\delta,\gamma,w} \quad (3r_D r_T^2 N_v) \quad (1459)$$

Raw expression

$${}^{21}R_{a,\epsilon} \leftarrow - \sum_{\gamma \in A} \sum_{i \in O} \sum_{j \in O} \sum_{k \in O} \sum_{b \in V} \sum_{c \in V} \sum_{d \in V} \frac{1}{2} {}^1T_{c,i} Y^{2,*}_{i,\epsilon} Z^*_{\epsilon,\gamma} Y^{3,*}_{b,\gamma} Y^{4,*}_{j,\gamma} {}^2D^{a,i,b,j} {}^2T_{d,j,b,k} V_{a,c,k,d} \quad (1460)$$

Factorized expression

$$\tau^0_{\gamma,\delta,w} = \sum_{a \in V} {}^2D^3_{a,w} Y^3_{a,\gamma} Y^{3,*}_{a,\delta} \quad (3r_D r_T^2 N_v) \quad (1461)$$

$$\tau^1_{\gamma,\delta,w} = \sum_{i \in O} {}^2D^4_{i,w} Y^4_{i,\gamma} Y^{4,*}_{i,\delta} \quad (3r_D r_T^2 N_o) \quad (1462)$$

$$\tau^2_{\gamma,\delta,w} = \sum_{\epsilon \in A} Z^*_{\delta,\epsilon} \tau^0_{\gamma,\epsilon,w} \tau^1_{\gamma,\epsilon,w} \quad (3r_D r_T^3) \quad (1463)$$

$$\tau^3_{\gamma,\delta,w} = \sum_{\epsilon \in A} Z_{\gamma,\epsilon} \tau^2_{\epsilon,\delta,w} \quad (2r_D r_T^3) \quad (1464)$$

$$\tau^4_{\alpha,i} = \sum_{a \in V} {}^1T_{a,i} W^4_{a,\alpha} \quad (2r_V N_o N_v) \quad (1465)$$

$$\tau^5_{\alpha,\beta} = \sum_{i \in O} W^1_{i,\alpha} \tau^4_{\beta,i} \quad (2r_V^2 N_o) \quad (1466)$$

$$\tau^6_{\alpha,i} = \sum_{\beta \in B} X_{\alpha,\beta} W^3_{i,\beta} \tau^5_{\alpha,\beta} \quad (3r_V^2 N_o) \quad (1467)$$

$$\tau^7_{i,j} = \sum_{\alpha \in B} W^2_{i,\alpha} \tau^6_{\alpha,j} \quad (2r_V N_o^2) \quad (1468)$$

$$\tau^8_{\gamma,i} = \sum_{j \in O} Y^2_{j,\gamma} \tau^7_{i,j} \quad (2r_T N_o^2) \quad (1469)$$

$$\tau^9_{\gamma,\delta,w} = \sum_{i \in O} {}^2D^2_{i,w} Y^{2,*}_{i,\delta} \tau^8_{\gamma,i} \quad (3r_D r_T^2 N_o) \quad (1470)$$

$${}^{21}R_{a,\gamma} \leftarrow \sum_{\delta \in A} \sum_{w \in D} \frac{1}{2} {}^2D^1_{a,w} Y^1_{a,\delta} \tau^3_{\delta,\gamma,w} \tau^9_{\delta,\gamma,w} \quad (4r_D r_T^2 N_v) \quad (1471)$$

Raw expression

$${}^{21}R_{a,\epsilon} \leftarrow - \sum_{\gamma \in A} \sum_{i \in O} \sum_{j \in O} \sum_{k \in O} \sum_{b \in V} \sum_{c \in V} \sum_{d \in V} \frac{1}{2} {}^1T_{c,i} Y^{2,*}_{i,\epsilon} Z^*_{\epsilon,\gamma} Y^{3,*}_{b,\gamma} Y^{4,*}_{j,\gamma} {}^2D^{a,i,b,j} {}^2T_{d,k,b,j} V_{a,d,k,c} \quad (1472)$$

Factorized expression

$$\tau^0_{\gamma,\delta,w} = \sum_{a \in V} {}^2D^3_{a,w} Y^1_{a,\gamma} Y^{3,*}_{a,\delta} \quad (3r_D r_T^2 N_v) \quad (1473)$$

$$\tau^1_{\gamma,\delta,w} = \sum_{i \in O} {}^2D^4_{i,w} Y^2_{i,\gamma} Y^{4,*}_{i,\delta} \quad (3r_D r_T^2 N_o) \quad (1474)$$

$$\tau^2_{\alpha,i} = \sum_{a \in V} {}^1T_{a,i} W^2_{a,\alpha} \quad (2r_V N_o N_v) \quad (1487)$$

$$\tau^2_{\gamma,\delta,w} = \sum_{\epsilon \in A} Z^*_{\delta,\epsilon} \tau^0_{\gamma,\epsilon,w} \tau^1_{\gamma,\epsilon,w} \quad (3r_D r_T^3) \quad (1475)$$

$$\tau^3_{\alpha,\beta} = \sum_{i \in O} W^3_{i,\beta} \tau^2_{\alpha,i} \quad (2r_V^2 N_o) \quad (1488)$$

$$\tau^3_{\gamma,\delta,w} = \sum_{\epsilon \in A} Z_{\epsilon,\gamma} \tau^2_{\epsilon,\delta,w} \quad (2r_D r_T^3) \quad (1476)$$

$$\tau^4_{\alpha,i} = \sum_{\beta \in B} X_{\alpha,\beta} W^4_{i,\beta} \tau^3_{\alpha,\beta} \quad (3r_V^2 N_o) \quad (1489)$$

$$\tau^4_{\alpha,i} = \sum_{a \in V} {}^1T_{a,i} W^4_{a,\alpha} \quad (2r_V N_o N_v) \quad (1477)$$

$$\tau^5_{i,j} = \sum_{\alpha \in B} W^1_{i,\alpha} \tau^4_{\alpha,j} \quad (2r_V N_o^2) \quad (1490)$$

$$\tau^5_{\alpha,\beta} = \sum_{i \in O} W^1_{i,\alpha} \tau^4_{\beta,i} \quad (2r_V^2 N_o) \quad (1478)$$

$$\tau^6_{\gamma,i} = \sum_{j \in O} Y^4_{j,\gamma} \tau^5_{j,i} \quad (2r_T N_o^2) \quad (1491)$$

$$\tau^6_{\alpha,i} = \sum_{\beta \in B} X_{\alpha,\beta} W^3_{i,\beta} \tau^5_{\alpha,\beta} \quad (3r_V^2 N_o) \quad (1479)$$

$$\tau^7_{\gamma,\delta,w} = \sum_{i \in O} {}^2D^4_{i,w} Y^{4,*}_{i,\delta} \tau^6_{\gamma,i} \quad (3r_D r_T^2 N_o) \quad (1492)$$

$$\tau^7_{i,j} = \sum_{\alpha \in B} W^2_{i,\alpha} \tau^6_{\alpha,j} \quad (2r_V N_o^2) \quad (1480)$$

$$\tau^8_{\gamma,\delta,w} = \sum_{\epsilon \in A} Z^*_{\delta,\epsilon} \tau^1_{\gamma,\epsilon,w} \tau^7_{\gamma,\epsilon,w} \quad (3r_D r_T^3) \quad (1493)$$

$$\tau^8_{\gamma,i} = \sum_{j \in O} Y^4_{j,\gamma} \tau^7_{i,j} \quad (2r_T N_o^2) \quad (1481)$$

$$\tau^9_{\gamma,\delta,w} = \sum_{\epsilon \in A} Z_{\gamma,\epsilon} \tau^8_{\epsilon,\delta,w} \quad (2r_D r_T^3) \quad (1494)$$

$$\tau^9_{\gamma,\delta,w} = \sum_{i \in O} {}^2D^2_{i,w} Y^{2,*}_{i,\delta} \tau^8_{\gamma,i} \quad (3r_D r_T^2 N_o) \quad (1482)$$

$${}^{21}R_{a,\gamma} \leftarrow \sum_{\delta \in A} \sum_{w \in D} \frac{1}{2} {}^2D^1_{a,w} Y^1_{a,\delta} \tau^0_{\delta,\gamma,w} \tau^9_{\delta,\gamma,w} \quad (4r_D r_T^2 N_v) \quad (1495)$$

$${}^{21}R_{a,\gamma} \leftarrow \sum_{\delta \in A} \sum_{w \in D} \frac{1}{2} {}^2D^1_{a,w} Y^3_{a,\delta} \tau^3_{\delta,\gamma,w} \tau^9_{\delta,\gamma,w} \quad (4r_D r_T^2 N_v) \quad \text{Raw expression} \quad (1483)$$

Raw expression

$${}^{21}R_{a,\epsilon} \leftarrow - \sum_{\gamma \in A} \sum_{i \in O} \sum_{j \in O} \sum_{k \in O} \sum_{b \in V} \sum_{c \in V} \sum_{d \in V} \frac{1}{2} {}^1T_{c,j} Y^{2,*}_{i,\epsilon} Z^*_{\epsilon,\gamma} Y^{3,*}_{b,\gamma} Y^{4,*}_{j,\gamma} {}^2D^{a,i,b,j} {}^2T_{a,i,d,k} V_{b,d,k,c} \quad (1484)$$

Factorized expression

$$\tau^0_{\gamma,\delta,w} = \sum_{i \in O} {}^2D^2_{i,w} Y^2_{i,\gamma} Y^{2,*}_{i,\delta} \quad (3r_D r_T^2 N_o) \quad (1485)$$

$$\tau^1_{\gamma,\delta,w} = \sum_{a \in V} {}^2D^3_{a,w} Y^3_{a,\gamma} Y^{3,*}_{a,\delta} \quad (3r_D r_T^2 N_v) \quad (1486)$$

$${}^{21}R_{a,\epsilon} \leftarrow - \sum_{\gamma \in A} \sum_{i \in O} \sum_{j \in O} \sum_{k \in O} \sum_{b \in V} \sum_{c \in V} \sum_{d \in V} \frac{1}{2} {}^1T_{c,j} Y^{2,*}_{i,\epsilon} Z^*_{\epsilon,\gamma} Y^{3,*}_{b,\gamma} Y^{4,*}_{j,\gamma} {}^2D^{a,i,b,j} {}^2T_{a,k,d,i} V_{b,c,k,d} \quad (1496)$$

Factorized expression

$$\tau^0_{\gamma,\delta,w} = \sum_{i \in O} {}^2D^2_{i,w} Y^4_{i,\gamma} Y^{2,*}_{i,\delta} \quad (3r_D r_T^2 N_o) \quad (1497)$$

$$\tau^1_{\gamma,\delta,w} = \sum_{a \in V} {}^2D^3_{a,w} Y^1_{a,\gamma} Y^{3,*}_{a,\delta} \quad (3r_D r_T^2 N_v) \quad (1498)$$

$$\tau^2_{\alpha,i} = \sum_{a \in V} {}^1T_{a,i} W^2_{a,\alpha} \quad (2r_V N_o N_v) \quad (1499)$$

$$\tau^3_{\alpha,\beta} = \sum_{i \in O} W^3_{i,\beta} \tau^2_{\alpha,i} \quad (2r_V^2 N_o) \quad (1500)$$

$$\tau^4_{\alpha,i} = \sum_{\beta \in B} X_{\alpha,\beta} W^4_{i,\beta} \tau^3_{\alpha,\beta} \quad (3r_V^2 N_o) \quad (1501)$$

$$\tau^5_{i,j} = \sum_{\alpha \in B} W^1_{i,\alpha} \tau^4_{\alpha,j} \quad (2r_V N_o^2) \quad (1502)$$

$$\tau^6_{\gamma,i} = \sum_{j \in O} Y^2_{j,\gamma} \tau^5_{j,i} \quad (2r_T N_o^2) \quad (1503)$$

$$\tau^7_{\gamma,\delta,w} = \sum_{i \in O} {}^2D^4_{i,w} Y^{4,*}_{i,\delta} \tau^6_{\gamma,i} \quad (3r_D r_T^2 N_o) \quad (1504)$$

$$\tau^8_{\gamma,\delta,w} = \sum_{\epsilon \in A} Z^*_{\delta,\epsilon} \tau^1_{\gamma,\epsilon,w} \tau^7_{\gamma,\epsilon,w} \quad (3r_D r_T^3) \quad (1505)$$

$$\tau^9_{\gamma,\delta,w} = \sum_{\epsilon \in A} Z_{\epsilon,\gamma} \tau^8_{\epsilon,\delta,w} \quad (2r_D r_T^3) \quad (1506)$$

$${}^{21}R_{a,\gamma} \leftarrow \sum_{\delta \in A} \sum_{w \in D} \frac{1}{2} {}^2D^1_{a,w} Y^3_{a,\delta} \tau^0_{\delta,\gamma,w} \tau^9_{\delta,\gamma,w} \quad (4r_D r_T^2 N_v) \quad (1507)$$

Raw expression

$${}^{21}R_{a,\epsilon} \leftarrow - \sum_{\gamma \in A} \sum_{i \in O} \sum_{j \in O} \sum_{k \in O} \sum_{b \in V} \sum_{c \in V} \sum_{d \in V} \frac{1}{2} {}^1T_{c,j} Y^{2,*}_{i,\epsilon} Z^*_{\epsilon,\gamma} Y^{3,*}_{b,\gamma} Y^{4,*}_{j,\gamma} {}^2D^{a,i,b,j} {}^2T_{b,k,d,i} V_{a,d,k,c} \quad (1508)$$

Factorized expression

$$\tau^0_{\gamma,\delta,w} = \sum_{a \in V} {}^2D^3_{a,w} Y^1_{a,\gamma} Y^{3,*}_{a,\delta} \quad (3r_D r_T^2 N_v) \quad (1509)$$

$$\tau^1_{\gamma,\delta,w} = \sum_{i \in O} {}^2D^4_{i,w} Y^2_{i,\gamma} Y^{4,*}_{i,\delta} \quad (3r_D r_T^2 N_o) \quad (1510)$$

$$\tau^2_{\gamma,\delta,w} = \sum_{\epsilon \in A} Z^*_{\delta,\epsilon} \tau^0_{\gamma,\epsilon,w} \tau^1_{\gamma,\epsilon,w} \quad (3r_D r_T^3) \quad (1511)$$

$$\tau^3_{\gamma,\delta,w} = \sum_{\epsilon \in A} Z_{\epsilon,\gamma} \tau^2_{\epsilon,\delta,w} \quad (2r_D r_T^3) \quad (1512)$$

$$\tau^4_{\gamma,\delta,w} = \sum_{i \in O} {}^2D^2_{i,w} Y^4_{i,\gamma} Y^{2,*}_{i,\delta} \quad (3r_D r_T^2 N_o) \quad (1513)$$

$$\tau^5_{\gamma,i} = \sum_{a \in V} Y^3_{a,\gamma} f_{i,a} \quad (2r_T N_o N_v) \quad (1514)$$

$$\tau^6_{\gamma,w,i} = \sum_{\delta \in A} \tau^5_{\delta,i} \tau^3_{\delta,\gamma,w} \tau^4_{\delta,\gamma,w} \quad (3r_D r_T^2 N_o) \quad (1515)$$

$${}^{21}R_{a,\gamma} \leftarrow - \sum_{w \in D} \sum_{i \in O} \frac{1}{2} {}^2D^1_{a,w} {}^1T_{a,i} \tau^6_{\gamma,w,i} \quad (3r_D r_T N_o N_v) \quad (1516)$$

Raw expression

$${}^{21}R_{a,\epsilon} \leftarrow - \sum_{\gamma \in A} \sum_{i \in O} \sum_{j \in O} \sum_{k \in O} \sum_{b \in V} \sum_{c \in V} \sum_{d \in V} \frac{1}{2} {}^1T_{c,j} Y^{2,*}_{i,\epsilon} Z^*_{\epsilon,\gamma} Y^{3,*}_{b,\gamma} Y^{4,*}_{j,\gamma} {}^2D^{a,i,b,j} {}^2T_{d,i,a,k} V_{b,c,k,d} \quad (1517)$$

Factorized expression

$$\tau^0_{\gamma,\delta,w} = \sum_{i \in O} {}^2D^2_{i,w} Y^2_{i,\gamma} Y^{2,*}_{i,\delta} \quad (3r_D r_T^2 N_o) \quad (1518)$$

$$\tau^1_{\gamma,\delta,w} = \sum_{a \in V} {}^2D^3_{a,w} Y^3_{a,\gamma} Y^{3,*}_{a,\delta} \quad (3r_D r_T^2 N_v) \quad (1519)$$

$$\tau^2_{\gamma,\delta,w} = \sum_{i \in O} {}^2D^4_{i,w} Y^4_{i,\gamma} Y^{4,*}_{i,\delta} \quad (3r_D r_T^2 N_o) \quad (1520)$$

$$\tau^3_{\gamma,\delta,w} = \sum_{\epsilon \in A} Z^*_{\delta,\epsilon} \tau^1_{\gamma,\epsilon,w} \tau^2_{\gamma,\epsilon,w} \quad (3r_D r_T^3) \quad (1521)$$

$$\tau^4_{\gamma,\delta,w} = \sum_{\epsilon \in A} Z_{\gamma,\epsilon} \tau^3_{\epsilon,\delta,w} \quad (2r_D r_T^3) \quad (1522)$$

$$\tau^5_{\gamma,i} = \sum_{a \in V} Y^1_{a,\gamma} f_{i,a} \quad (2r_T N_o N_v) \quad (1523)$$

$$\tau^6_{\gamma,w,i} = \sum_{\delta \in A} \tau^5_{\delta,i} \tau^0_{\delta,\gamma,w} \tau^4_{\delta,\gamma,w} \quad (3r_D r_T^2 N_o) \quad (1524)$$

$${}^{21}R_{a,\gamma} \leftarrow - \sum_{w \in D} \sum_{i \in O} \frac{1}{2} {}^2D^1_{a,w} {}^1T_{a,i} \tau^6_{\gamma,w,i} \quad (3r_D r_T N_o N_v) \quad (1525)$$

Raw expression

$${}^{21}R_{a,\epsilon} \leftarrow - \sum_{\gamma \in A} \sum_{i \in O} \sum_{j \in O} \sum_{k \in O} \sum_{b \in V} \sum_{c \in V} \sum_{d \in V} \frac{1}{2} {}^1T_{c,j} Y^{2,*}_{i,\epsilon} Z^*_{\epsilon,\gamma} Y^{3,*}_{b,\gamma} Y^{4,*}_{j,\gamma} {}^2D^{a,i,b,j} {}^2T_{d,i,b,k} V_{a,d,k,c} \quad (1526)$$

$$\tau^2_{\gamma,w,i} = \sum_{a \in V} {}^2D^3_{a,w} {}^1T_{a,i} Y^{3,*}_{a,\gamma} \quad (3r_D r_T N_o N_v) \quad (1538)$$

Factorized expression

$$\tau^0_{\gamma,\delta,w} = \sum_{i \in O} {}^2D^2_{i,w} Y^2_{i,\gamma} Y^{2,*}_{i,\delta} \quad (3r_D r_T^2 N_o) \quad (1527)$$

$$\tau^1_{\gamma,\delta,w} = \sum_{i \in O} {}^2D^4_{i,w} Y^4_{i,\gamma} Y^{4,*}_{i,\delta} \quad (3r_D r_T^2 N_o) \quad (1528)$$

$$\tau^2_{\gamma,w,i} = \sum_{a \in V} {}^2D^3_{a,w} {}^1T_{a,i} Y^{3,*}_{a,\gamma} \quad (3r_D r_T N_o N_v) \quad (1529)$$

$$\tau^3_{\gamma,i} = \sum_{a \in V} Y^1_{a,\gamma} f_{i,a} \quad (2r_T N_o N_v) \quad (1539)$$

$$\tau^4_{\gamma,\delta,w} = \sum_{i \in O} \tau^3_{\gamma,i} \tau^2_{\delta,w,i} \quad (2r_D r_T^2 N_o) \quad (1540)$$

$$\tau^5_{\gamma,\delta,w} = \sum_{\epsilon \in A} Z^*_{\delta,\epsilon} \tau^1_{\gamma,\epsilon,w} \tau^4_{\gamma,\epsilon,w} \quad (3r_D r_T^3) \quad (1541)$$

$$\tau^6_{\gamma,\delta,w} = \sum_{\epsilon \in A} Z_{\epsilon,\gamma} \tau^5_{\epsilon,\delta,w} \quad (2r_D r_T^3) \quad (1542)$$

$$\tau^3_{\gamma,i} = \sum_{a \in V} Y^3_{a,\gamma} f_{i,a} \quad (2r_T N_o N_v) \quad (1530)$$

$${}^{21}R_{a,\gamma} \leftarrow - \sum_{\delta \in A} \sum_{w \in D} \frac{1}{2} {}^2D^1_{a,w} Y^3_{a,\delta} \tau^0_{\delta,\gamma,w} \tau^6_{\delta,\gamma,w} \quad (4r_D r_T^2 N_v) \quad (1543)$$

$$\tau^4_{\gamma,\delta,w} = \sum_{i \in O} \tau^3_{\gamma,i} \tau^2_{\delta,w,i} \quad (2r_D r_T^2 N_o) \quad (1531)$$

$$\tau^5_{\gamma,\delta,w} = \sum_{\epsilon \in A} Z^*_{\delta,\epsilon} \tau^1_{\gamma,\epsilon,w} \tau^4_{\gamma,\epsilon,w} \quad (3r_D r_T^3) \quad (1532)$$

$$\tau^6_{\gamma,\delta,w} = \sum_{\epsilon \in A} Z_{\gamma,\epsilon} \tau^5_{\epsilon,\delta,w} \quad (2r_D r_T^3) \quad (1533)$$

$${}^{21}R_{a,\gamma} \leftarrow - \sum_{\delta \in A} \sum_{w \in D} \frac{1}{2} {}^2D^1_{a,w} Y^1_{a,\delta} \tau^0_{\delta,\gamma,w} \tau^6_{\delta,\gamma,w} \quad (4r_D r_T^2 N_v) \quad (1534)$$

Raw expression

$${}^{21}R_{a,\epsilon} \leftarrow - \sum_{\gamma \in A} \sum_{i \in O} \sum_{j \in O} \sum_{k \in O} \sum_{b \in V} \sum_{c \in V} \sum_{d \in V} \frac{1}{2} {}^1T_{c,j} Y^{2,*}_{i,\epsilon} Z^*_{\epsilon,\gamma} Y^{3,*}_{b,\gamma} Y^{4,*}_{j,\gamma} {}^2D^{a,i,b,j} {}^2T_{d,k,a,i} V_{b,d,k,c} \quad (1535)$$

Factorized expression

$$\tau^0_{\gamma,\delta,w} = \sum_{i \in O} {}^2D^2_{i,w} Y^4_{i,\gamma} Y^{2,*}_{i,\delta} \quad (3r_D r_T^2 N_o) \quad (1536)$$

$$\tau^1_{\gamma,\delta,w} = \sum_{i \in O} {}^2D^4_{i,w} Y^2_{i,\gamma} Y^{4,*}_{i,\delta} \quad (3r_D r_T^2 N_o) \quad (1537)$$

Raw expression

$${}^{21}R_{a,\epsilon} \leftarrow - \sum_{\gamma \in A} \sum_{i \in O} \sum_{j \in O} \sum_{k \in O} \sum_{b \in V} \sum_{c \in V} \sum_{d \in V} \frac{1}{2} {}^1T_{c,k} Y^{2,*}_{i,\epsilon} Z^*_{\epsilon,\gamma} Y^{3,*}_{b,\gamma} Y^{4,*}_{j,\gamma} {}^2D^{a,i,b,j} {}^2T_{a,i,d,j} V_{b,c,k,d} \quad (1544)$$

Factorized expression

$$\tau^0_{i,j} = \sum_{a \in V} {}^1T_{a,i} f_{j,a} \quad (2N_o^2 N_v) \quad (1545)$$

$$\tau^1_{\gamma,i} = \sum_{j \in O} Y^2_{j,\gamma} \tau^0_{i,j} \quad (2r_T N_o^2) \quad (1546)$$

$$\tau^2_{\gamma,\delta,w} = \sum_{i \in O} {}^2D^2_{i,w} Y^{2,*}_{i,\delta} \tau^1_{\gamma,i} \quad (3r_D r_T^2 N_o) \quad (1547)$$

$$\tau^3_{\gamma,\delta,w} = \sum_{a \in V} {}^2D^3_{a,w} Y^3_{a,\gamma} Y^{3,*}_{a,\delta} \quad (3r_D r_T^2 N_v) \quad (1548)$$

$$\tau^4_{\gamma,\delta,w} = \sum_{i \in O} {}^2D^4_{i,w} Y^4_{i,\gamma} Y^{4,*}_{i,\delta} \quad (3r_D r_T^2 N_o) \quad (1549)$$

$$\tau^5_{\gamma,\delta,w} = \sum_{\epsilon \in A} Z^*_{\delta,\epsilon} \tau^3_{\gamma,\epsilon,w} \tau^4_{\gamma,\epsilon,w} \quad (3r_D r_T^3) \quad (1550)$$

Factorized expression

$$\tau_{\gamma,\delta,w}^6 = \sum_{\epsilon \in A} Z_{\gamma,\epsilon} \tau_{\epsilon,\delta,w}^5 \quad (2r_D r_T^3) \quad (1551)$$

$$\tau_{\gamma,\delta,w}^0 = \sum_{i \in O} {}^2D_{i,w}^2 Y_{i,\gamma}^2 Y_{i,\delta}^{2,*} \quad (3r_D r_T^2 N_o) \quad (1563)$$

$${}^{21}R_{a,\gamma} \leftarrow - \sum_{\delta \in A} \sum_{w \in D} \frac{1}{2} {}^2D_{a,w}^1 Y_{a,\delta}^1 \tau_{\delta,\gamma,w}^2 \tau_{\delta,\gamma,w}^6 \quad (4r_D r_T^2 N_v) \quad (1552)$$

$$\tau_{\gamma,\delta,w}^1 = \sum_{a \in V} {}^2D_{a,w}^3 Y_{a,\gamma}^3 Y_{a,\delta}^{3,*} \quad (3r_D r_T^2 N_v) \quad (1564)$$

Raw expression

$${}^{21}R_{a,\epsilon} \leftarrow - \sum_{\gamma \in A} \sum_{i \in O} \sum_{j \in O} \sum_{k \in O} \sum_{b \in V} \sum_{c \in V} \sum_{d \in V} \frac{1}{2} {}^1T_{c,k} Y_{i,\epsilon}^{2,*} Z_{\epsilon,\gamma}^* Y_{b,\gamma}^{3,*} Y_{j,\gamma}^{4,*} {}^2D_{a,i,b,j} {}^2T_{b,j,d,i} V_{a,c,k,d} \quad (1553)$$

$$\tau_{i,j}^2 = \sum_{a \in V} {}^1T_{a,i} f_{j,a} \quad (2N_o^2 N_v) \quad (1565)$$

$$\tau_{\gamma,i}^3 = \sum_{j \in O} Y_{j,\gamma}^4 \tau_{i,j}^2 \quad (2r_T N_o^2) \quad (1566)$$

Factorized expression

$$\tau_{\gamma,\delta,w}^0 = \sum_{a \in V} {}^2D_{a,w}^3 Y_{a,\gamma}^1 Y_{a,\delta}^{3,*} \quad (3r_D r_T^2 N_v) \quad (1554)$$

$$\tau_{\gamma,\delta,w}^4 = \sum_{i \in O} {}^2D_{i,w}^4 Y_{i,\delta}^{4,*} \tau_{\gamma,i}^3 \quad (3r_D r_T^2 N_o) \quad (1567)$$

$$\tau_{\gamma,\delta,w}^1 = \sum_{i \in O} {}^2D_{i,w}^4 Y_{i,\gamma}^2 Y_{i,\delta}^{4,*} \quad (3r_D r_T^2 N_o) \quad (1555)$$

$$\tau_{\gamma,\delta,w}^5 = \sum_{\epsilon \in A} Z_{\delta,\epsilon}^* \tau_{\gamma,\epsilon,w}^1 \tau_{\gamma,\epsilon,w}^4 \quad (3r_D r_T^3) \quad (1568)$$

$$\tau_{\gamma,\delta,w}^2 = \sum_{\epsilon \in A} Z_{\delta,\epsilon}^* \tau_{\gamma,\epsilon,w}^0 \tau_{\gamma,\epsilon,w}^1 \quad (3r_D r_T^3) \quad (1556)$$

$$\tau_{\gamma,\delta,w}^6 = \sum_{\epsilon \in A} Z_{\gamma,\epsilon} \tau_{\epsilon,\delta,w}^5 \quad (2r_D r_T^3) \quad (1569)$$

$$\tau_{\gamma,\delta,w}^3 = \sum_{\epsilon \in A} Z_{\epsilon,\gamma} \tau_{\epsilon,\delta,w}^2 \quad (2r_D r_T^3) \quad (1557)$$

$${}^{21}R_{a,\gamma} \leftarrow - \sum_{\delta \in A} \sum_{w \in D} \frac{1}{2} {}^2D_{a,w}^1 Y_{a,\delta}^1 \tau_{\delta,\gamma,w}^0 \tau_{\delta,\gamma,w}^6 \quad (4r_D r_T^2 N_v) \quad (1570)$$

Raw expression

$$\tau_{i,j}^4 = \sum_{a \in V} {}^1T_{a,i} f_{j,a} \quad (2N_o^2 N_v) \quad (1558)$$

$${}^{21}R_{a,\epsilon} \leftarrow - \sum_{\gamma \in A} \sum_{i \in O} \sum_{j \in O} \sum_{k \in O} \sum_{b \in V} \sum_{c \in V} \sum_{d \in V} \frac{1}{2} {}^1T_{c,k} Y_{i,\epsilon}^{2,*} Z_{\epsilon,\gamma}^* Y_{b,\gamma}^{3,*} Y_{j,\gamma}^{4,*} {}^2D_{a,i,b,j} {}^2T_{d,j,a,i} V_{b,c,k,d} \quad (1571)$$

$$\tau_{\gamma,i}^5 = \sum_{j \in O} Y_{j,\gamma}^4 \tau_{i,j}^4 \quad (2r_T N_o^2) \quad (1559)$$

Factorized expression

$$\tau_{\gamma,\delta,w}^6 = \sum_{i \in O} {}^2D_{i,w}^2 Y_{i,\delta}^{2,*} \tau_{\gamma,i}^5 \quad (3r_D r_T^2 N_o) \quad (1560)$$

$$\tau_{\gamma,\delta,w}^0 = \sum_{i \in O} {}^2D_{i,w}^2 Y_{i,\gamma}^4 Y_{i,\delta}^{2,*} \quad (3r_D r_T^2 N_o) \quad (1572)$$

$${}^{21}R_{a,\gamma} \leftarrow - \sum_{\delta \in A} \sum_{w \in D} \frac{1}{2} {}^2D_{a,w}^1 Y_{a,\delta}^3 \tau_{\delta,\gamma,w}^3 \tau_{\delta,\gamma,w}^6 \quad (4r_D r_T^2 N_v) \quad (1561)$$

$$\tau_{\gamma,\delta,w}^1 = \sum_{a \in V} {}^2D_{a,w}^3 Y_{a,\gamma}^1 Y_{a,\delta}^{3,*} \quad (3r_D r_T^2 N_v) \quad (1573)$$

Raw expression

$${}^{21}R_{a,\epsilon} \leftarrow - \sum_{\gamma \in A} \sum_{i \in O} \sum_{j \in O} \sum_{k \in O} \sum_{b \in V} \sum_{c \in V} \sum_{d \in V} \frac{1}{2} {}^1T_{c,k} Y_{i,\epsilon}^{2,*} Z_{\epsilon,\gamma}^* Y_{b,\gamma}^{3,*} Y_{j,\gamma}^{4,*} {}^2D_{a,i,b,j} {}^2T_{d,i,b,j} V_{a,c,k,d} \quad (1562)$$

$$\tau_{i,j}^2 = \sum_{a \in V} {}^1T_{a,i} f_{j,a} \quad (2N_o^2 N_v) \quad (1574)$$

$$\tau_{\gamma,i}^3 = \sum_{j \in O} Y_{j,\gamma}^2 \tau_{i,j}^2 \quad (2r_T N_o^2) \quad (1575)$$

$$\tau^4_{\gamma,\delta,w} = \sum_{i \in O} {}^2D^4_{i,w} Y^{4,*}_{i,\delta} \tau^3_{\gamma,i} \quad (3r_D r_T^2 N_o) \quad (1576)$$

$$\tau^5_{\gamma,\delta,w} = \sum_{\epsilon \in A} Z^*_{\delta,\epsilon} \tau^1_{\gamma,\epsilon,w} \tau^4_{\gamma,\epsilon,w} \quad (3r_D r_T^3) \quad (1577)$$

$$\tau^6_{\gamma,\delta,w} = \sum_{\epsilon \in A} Z_{\epsilon,\gamma} \tau^5_{\epsilon,\delta,w} \quad (2r_D r_T^3) \quad (1578)$$

$${}^{21}R_{a,\gamma} \leftarrow - \sum_{\delta \in A} \sum_{w \in D} \frac{1}{2} {}^2D^1_{a,w} Y^3_{a,\delta} \tau^0_{\delta,\gamma,w} \tau^6_{\delta,\gamma,w} \quad (4r_D r_T^2 N_v) \quad (1579)$$

### G. Contributions from $(H^1 T^1 T^1 T^1 T)_c$

Raw expression

$${}^{21}R_{a,\epsilon} \leftarrow \sum_{\gamma \in A} \sum_{i \in O} \sum_{j \in O} \sum_{k \in O} \sum_{l \in O} \sum_{b \in V} \sum_{c \in V} \sum_{d \in V} {}^1T_{a,k} {}^1T_{b,l} {}^1T_{c,i} {}^1T_{d,j} Y^{2,*}_{i,\epsilon} Z^*_{\epsilon,\gamma} Y^{3,*}_{b,\gamma} Y^{4,*}_{j,\gamma} {}^2D^{a,i,b,j} V_{k,c,l,d} \quad (1580)$$

Factorized expression

$$\tau^0_{\alpha,i} = \sum_{a \in V} {}^1T_{a,i} W^2_{a,\alpha} \quad (2r_V N_o N_v) \quad (1581)$$

$$\tau^1_{\gamma,\alpha,w} = \sum_{i \in O} {}^2D^2_{i,w} Y^{2,*}_{i,\gamma} \tau^0_{\alpha,i} \quad (3r_D r_T r_V N_o) \quad (1582)$$

$$\tau^2_{\alpha,i} = \sum_{a \in V} {}^1T_{a,i} W^4_{a,\alpha} \quad (2r_V N_o N_v) \quad (1583)$$

$$\tau^3_{\gamma,\alpha,w} = \sum_{i \in O} {}^2D^4_{i,w} Y^{4,*}_{i,\gamma} \tau^2_{\alpha,i} \quad (3r_D r_T r_V N_o) \quad (1584)$$

$$\tau^4_{\gamma,w,i} = \sum_{a \in V} {}^2D^3_{a,w} {}^1T_{a,i} Y^{3,*}_{a,\gamma} \quad (3r_D r_T N_o N_v) \quad (1585)$$

$$\tau^5_{\gamma,\alpha,w} = \sum_{i \in O} W^3_{i,\alpha} \tau^4_{\gamma,w,i} \quad (2r_D r_T r_V N_o) \quad (1586)$$

$$\tau^6_{\gamma,\alpha,w} = \sum_{\beta \in B} X_{\alpha,\beta} \tau^3_{\gamma,\beta,w} \tau^5_{\gamma,\beta,w} \quad (3r_D r_T r_V^2) \quad (1587)$$

$$\tau^7_{\gamma,\alpha,w} = \sum_{\delta \in A} Z^*_{\gamma,\delta} \tau^6_{\delta,\alpha,w} \quad (2r_D r_T^2 r_V) \quad (1588)$$

$$\tau^8_{\gamma,w,i} = \sum_{\alpha \in B} W^1_{i,\alpha} \tau^1_{\gamma,\alpha,w} \tau^7_{\gamma,\alpha,w} \quad (3r_D r_T r_V N_o) \quad (1589)$$

$${}^{21}R_{a,\gamma} \leftarrow \sum_{w \in D} \sum_{i \in O} {}^2D^1_{a,w} {}^1T_{a,i} \tau^8_{\gamma,w,i} \quad (3r_D r_T N_o N_v) \quad (1590)$$

### H. Contributions from $(H^1 T^1 T^2 T)_c$

Raw expression

$${}^{21}R_{a,\epsilon} \leftarrow \sum_{\gamma \in A} \sum_{i \in O} \sum_{j \in O} \sum_{k \in O} \sum_{l \in O} \sum_{b \in V} \sum_{c \in V} \sum_{d \in V} \frac{1}{2} {}^1T_{a,k} {}^1T_{b,l} Y^{2,*}_{i,\epsilon} Z^*_{\epsilon,\gamma} Y^{3,*}_{b,\gamma} Y^{4,*}_{j,\gamma} {}^2D^{a,i,b,j} {}^2T_{c,i,d,j} V_{k,c,l,d} \quad (1591)$$

Factorized expression

$$\tau^0_{\gamma,\alpha} = \sum_{a \in V} W^4_{a,\alpha} Y^3_{a,\gamma} \quad (2r_T r_V N_v) \quad (1592)$$

$$\tau^1_{\gamma,\alpha} = \sum_{i \in O} W^3_{i,\alpha} Y^4_{i,\gamma} \quad (2r_T r_V N_o) \quad (1593)$$

$$\tau^2_{\gamma,\alpha} = \sum_{\beta \in B} X_{\alpha,\beta} \tau^0_{\gamma,\beta} \tau^1_{\gamma,\beta} \quad (3r_T r_V^2) \quad (1594)$$

$$\tau^3_{\gamma,\alpha} = \sum_{\delta \in A} Z_{\gamma,\delta} \tau^2_{\delta,\alpha} \quad (2r_T^2 r_V) \quad (1595)$$

$$\tau^4_{\gamma,\delta,w} = \sum_{a \in V} {}^2D^3_{a,w} Y^1_{a,\gamma} Y^{3,*}_{a,\delta} \quad (3r_D r_T^2 N_v) \quad (1596)$$

$$\tau^5_{\gamma,\delta,w} = \sum_{i \in O} {}^2D^4_{i,w} Y^2_{i,\gamma} Y^{4,*}_{i,\delta} \quad (3r_D r_T^2 N_o) \quad (1597)$$

$$\tau^6_{\gamma,\delta,w} = \sum_{\epsilon \in A} Z^*_{\delta,\epsilon} \tau^4_{\gamma,\epsilon,w} \tau^5_{\gamma,\epsilon,w} \quad (3r_D r_T^3) \quad (1598)$$

$$\tau^7_{\gamma,\alpha,w} = \sum_{\delta \in A} \tau^3_{\delta,\alpha} \tau^6_{\delta,\gamma,w} \quad (2r_D r_T^2 r_V) \quad (1599)$$



$$\tau_{\alpha,i}^8 = \sum_{a \in V} {}^1T_{a,i} W_{a,\alpha}^2 \quad (2r_V N_o N_v) \quad (1600)$$

$$\tau_{\alpha,i}^8 = \sum_{a \in V} {}^1T_{a,i} W_{a,\alpha}^2 \quad (2r_V N_o N_v) \quad (1613)$$

$$\tau_{\gamma,\alpha,w}^9 = \sum_{i \in O} {}^2D_{i,w}^2 Y_{i,\gamma}^{2,*} \tau_{\alpha,i}^8 \quad (3r_D r_T r_V N_o) \quad (1601)$$

$$\tau_{\gamma,\alpha,w}^9 = \sum_{i \in O} {}^2D_{i,w}^2 Y_{i,\gamma}^{2,*} \tau_{\alpha,i}^8 \quad (3r_D r_T r_V N_o) \quad (1614)$$

$$\tau_{\gamma,w,i}^{10} = \sum_{\alpha \in B} W_{i,\alpha}^1 \tau_{\gamma,\alpha,w}^7 \tau_{\gamma,\alpha,w}^9 \quad (3r_D r_T r_V N_o) \quad (1602)$$

$$\tau_{\gamma,w,i}^{10} = \sum_{\alpha \in B} W_{i,\alpha}^1 \tau_{\gamma,\alpha,w}^7 \tau_{\gamma,\alpha,w}^9 \quad (3r_D r_T r_V N_o) \quad (1615)$$

$${}^{21}R_{a,\gamma} \leftarrow - \sum_{w \in D} \sum_{i \in O} {}^2D_{a,w}^1 {}^1T_{a,i} \tau_{\gamma,w,i}^{10} \quad (3r_D r_T N_o N_v) \quad (1603)$$

$${}^{21}R_{a,\gamma} \leftarrow - \sum_{w \in D} \sum_{i \in O} {}^2D_{a,w}^1 {}^1T_{a,i} \tau_{\gamma,w,i}^{10} \quad (3r_D r_T N_o N_v) \quad (1616)$$

Raw expression

$${}^{21}R_{a,\epsilon} \leftarrow \sum_{\gamma \in A} \sum_{i \in O} \sum_{j \in O} \sum_{k \in O} \sum_{l \in O} \sum_{b \in V} \sum_{c \in V} \sum_{d \in V} \frac{1}{2} \quad (1604)$$

$${}^1T_{a,k} {}^1T_{b,l} Y_{i,\epsilon}^{2,*} Z_{\epsilon,\gamma}^* Y_{b,\gamma}^{3,*} Y_{j,\gamma}^{4,*} {}^2D_{a,i,b,j} {}^2T_{c,j,d,i} V_{k,d,l,c}$$

Raw expression

$${}^{21}R_{a,\epsilon} \leftarrow \sum_{\gamma \in A} \sum_{i \in O} \sum_{j \in O} \sum_{k \in O} \sum_{l \in O} \sum_{b \in V} \sum_{c \in V} \sum_{d \in V} \frac{1}{2} \quad (1617)$$

$${}^1T_{a,k} {}^1T_{c,i} Y_{i,\epsilon}^{2,*} Z_{\epsilon,\gamma}^* Y_{b,\gamma}^{3,*} Y_{j,\gamma}^{4,*} {}^2D_{a,i,b,j} {}^2T_{b,j,d,l} V_{k,d,l,c}$$

Factorized expression

$$\tau_{\gamma,\delta,w}^0 = \sum_{a \in V} {}^2D_{a,w}^3 Y_{a,\gamma}^3 Y_{a,\delta}^{3,*} \quad (3r_D r_T^2 N_v) \quad (1605)$$

$$\tau_{\gamma,\delta,w}^0 = \sum_{a \in V} {}^2D_{a,w}^3 Y_{a,\gamma}^1 Y_{a,\delta}^{3,*} \quad (3r_D r_T^2 N_v) \quad (1618)$$

$$\tau_{\gamma,\delta,w}^1 = \sum_{i \in O} {}^2D_{i,w}^4 Y_{i,\gamma}^4 Y_{i,\delta}^{4,*} \quad (3r_D r_T^2 N_o) \quad (1606)$$

$$\tau_{\gamma,\delta,w}^1 = \sum_{i \in O} {}^2D_{i,w}^4 Y_{i,\gamma}^2 Y_{i,\delta}^{4,*} \quad (3r_D r_T^2 N_o) \quad (1619)$$

$$\tau_{\gamma,\delta,w}^2 = \sum_{\epsilon \in A} Z_{\delta,\epsilon}^* \tau_{\gamma,\epsilon,w}^0 \tau_{\gamma,\epsilon,w}^1 \quad (3r_D r_T^3) \quad (1607)$$

$$\tau_{\gamma,\delta,w}^2 = \sum_{\epsilon \in A} Z_{\delta,\epsilon}^* \tau_{\gamma,\epsilon,w}^0 \tau_{\gamma,\epsilon,w}^1 \quad (3r_D r_T^3) \quad (1620)$$

$$\tau_{\gamma,\alpha}^3 = \sum_{a \in V} W_{a,\alpha}^4 Y_{a,\gamma}^1 \quad (2r_T r_V N_v) \quad (1608)$$

$$\tau_{\gamma,\delta,w}^3 = \sum_{\epsilon \in A} Z_{\epsilon,\gamma} \tau_{\epsilon,\delta,w}^2 \quad (2r_D r_T^3) \quad (1621)$$

$$\tau_{\gamma,\alpha}^4 = \sum_{i \in O} W_{i,\alpha}^3 Y_{i,\gamma}^2 \quad (2r_T r_V N_o) \quad (1609)$$

$$\tau_{\gamma,\delta,w}^4 = \sum_{i \in O} {}^2D_{i,w}^2 Y_{i,\gamma}^4 Y_{i,\delta}^{2,*} \quad (3r_D r_T^2 N_o) \quad (1622)$$

$$\tau_{\gamma,\alpha}^5 = \sum_{\beta \in B} X_{\alpha,\beta} \tau_{\gamma,\beta}^3 \tau_{\gamma,\beta}^4 \quad (3r_T r_V^2) \quad (1610)$$

$$\tau_{\alpha,i}^5 = \sum_{a \in V} {}^1T_{a,i} W_{a,\alpha}^4 \quad (2r_V N_o N_v) \quad (1623)$$

$$\tau_{\gamma,\alpha}^6 = \sum_{\delta \in A} Z_{\delta,\gamma} \tau_{\delta,\alpha}^5 \quad (2r_T^2 r_V) \quad (1611)$$

$$\tau_{\alpha}^6 = \sum_{i \in O} W_{i,\alpha}^3 \tau_{\alpha,i}^5 \quad (2r_V N_o) \quad (1624)$$

$$\tau_{\gamma,\alpha,w}^7 = \sum_{\delta \in A} \tau_{\delta,\alpha}^6 \tau_{\delta,\gamma,w}^2 \quad (2r_D r_T^2 r_V) \quad (1612)$$

$$\tau_{\alpha}^7 = \sum_{\beta \in B} \tau_{\beta}^6 X_{\alpha,\beta} \quad (2r_V^2) \quad (1625)$$

$$\tau^8_{i,a} = \sum_{\alpha \in B} \tau^7_{\alpha} W^1_{i,\alpha} W^2_{a,\alpha} \quad (3r_V N_o N_v) \quad (1626)$$

$$\tau^9_{\gamma,i} = \sum_{a \in V} Y^3_{a,\gamma} \tau^8_{i,a} \quad (2r_T N_o N_v) \quad (1627)$$

$$\tau^{10}_{\gamma,w,i} = \sum_{\delta \in A} \tau^9_{\delta,i} \tau^3_{\delta,\gamma,w} \tau^4_{\delta,\gamma,w} \quad (3r_D r_T^2 N_o) \quad (1628)$$

$${}^{21}R_{a,\gamma} \leftarrow - \sum_{w \in D} \sum_{i \in O} {}^2D^1_{a,w} {}^1T_{a,i} \tau^{10}_{\gamma,w,i} \quad (3r_D r_T N_o N_v) \quad (1629)$$

Raw expression

$${}^{21}R_{a,\epsilon} \leftarrow \sum_{\gamma \in A} \sum_{i \in O} \sum_{j \in O} \sum_{k \in O} \sum_{l \in O} \sum_{b \in V} \sum_{c \in V} \sum_{d \in V} \frac{1}{2} \quad (1630)$$

$${}^1T_{a,k} {}^1T_{c,i} Y^{2,*}_{i,\epsilon} Z^{*}_{\epsilon,\gamma} Y^{3,*}_{b,\gamma} Y^{4,*}_{j,\gamma} {}^2D^{a,i,b,j} {}^2T_{b,l,d,j} V_{k,c,l,d}$$

Factorized expression

$$\tau^0_{\gamma,\delta,w} = \sum_{i \in O} {}^2D^2_{i,w} Y^2_{i,\gamma} Y^{2,*}_{i,\delta} \quad (3r_D r_T^2 N_o) \quad (1631)$$

$$\tau^1_{\gamma,\delta,w} = \sum_{a \in V} {}^2D^3_{a,w} Y^3_{a,\gamma} Y^{3,*}_{a,\delta} \quad (3r_D r_T^2 N_v) \quad (1632)$$

$$\tau^2_{\gamma,\delta,w} = \sum_{i \in O} {}^2D^4_{i,w} Y^4_{i,\gamma} Y^{4,*}_{i,\delta} \quad (3r_D r_T^2 N_o) \quad (1633)$$

$$\tau^3_{\gamma,\delta,w} = \sum_{\epsilon \in A} Z^{*}_{\delta,\epsilon} \tau^1_{\gamma,\epsilon,w} \tau^2_{\gamma,\epsilon,w} \quad (3r_D r_T^3) \quad (1634)$$

$$\tau^4_{\gamma,\delta,w} = \sum_{\epsilon \in A} Z_{\gamma,\epsilon} \tau^3_{\epsilon,\delta,w} \quad (2r_D r_T^3) \quad (1635)$$

$$\tau^5_{\alpha,i} = \sum_{a \in V} {}^1T_{a,i} W^4_{a,\alpha} \quad (2r_V N_o N_v) \quad (1636)$$

$$\tau^6_{\alpha} = \sum_{i \in O} W^3_{i,\alpha} \tau^5_{\alpha,i} \quad (2r_V N_o) \quad (1637)$$

$$\tau^7_{\alpha} = \sum_{\beta \in B} \tau^6_{\beta} X_{\alpha,\beta} \quad (2r_V^2) \quad (1638)$$

$$\tau^8_{i,a} = \sum_{\alpha \in B} \tau^7_{\alpha} W^1_{i,\alpha} W^2_{a,\alpha} \quad (3r_V N_o N_v) \quad (1639)$$

$$\tau^9_{\gamma,i} = \sum_{a \in V} Y^1_{a,\gamma} \tau^8_{i,a} \quad (2r_T N_o N_v) \quad (1640)$$

$$\tau^{10}_{\gamma,w,i} = \sum_{\delta \in A} \tau^9_{\delta,i} \tau^0_{\delta,\gamma,w} \tau^4_{\delta,\gamma,w} \quad (3r_D r_T^2 N_o) \quad (1641)$$

$${}^{21}R_{a,\gamma} \leftarrow - \sum_{w \in D} \sum_{i \in O} {}^2D^1_{a,w} {}^1T_{a,i} \tau^{10}_{\gamma,w,i} \quad (3r_D r_T N_o N_v) \quad (1642)$$

Raw expression

$${}^{21}R_{a,\epsilon} \leftarrow \sum_{\gamma \in A} \sum_{i \in O} \sum_{j \in O} \sum_{k \in O} \sum_{l \in O} \sum_{b \in V} \sum_{c \in V} \sum_{d \in V} \frac{1}{2} \quad (1643)$$

$${}^1T_{a,k} {}^1T_{c,i} Y^{2,*}_{i,\epsilon} Z^{*}_{\epsilon,\gamma} Y^{3,*}_{b,\gamma} Y^{4,*}_{j,\gamma} {}^2D^{a,i,b,j} {}^2T_{d,j,b,l} V_{k,c,l,d}$$

Factorized expression

$$\tau^0_{\gamma,\delta,w} = \sum_{i \in O} {}^2D^2_{i,w} Y^2_{i,\gamma} Y^{2,*}_{i,\delta} \quad (3r_D r_T^2 N_o) \quad (1644)$$

$$\tau^1_{\alpha,i} = \sum_{a \in V} {}^1T_{a,i} W^2_{a,\alpha} \quad (2r_V N_o N_v) \quad (1645)$$

$$\tau^2_{\gamma,\alpha,w} = \sum_{i \in O} {}^2D^4_{i,w} Y^{4,*}_{i,\gamma} \tau^1_{\alpha,i} \quad (3r_D r_T r_V N_o) \quad (1646)$$

$$\tau^3_{\gamma,w,i} = \sum_{a \in V} {}^2D^3_{a,w} {}^1T_{a,i} Y^{3,*}_{a,\gamma} \quad (3r_D r_T N_o N_v) \quad (1647)$$

$$\tau^4_{\gamma,\alpha,w} = \sum_{i \in O} W^1_{i,\alpha} \tau^3_{\gamma,w,i} \quad (2r_D r_T r_V N_o) \quad (1648)$$

$$\tau^5_{\gamma,\alpha} = \sum_{a \in V} W^4_{a,\alpha} Y^3_{a,\gamma} \quad (2r_T r_V N_v) \quad (1649)$$

$$\tau^6_{\gamma,\alpha} = \sum_{i \in O} W^3_{i,\alpha} Y^4_{i,\gamma} \quad (2r_T r_V N_o) \quad (1650)$$

$$\tau^7_{\gamma,\alpha} = \sum_{\beta \in B} X_{\alpha,\beta} \tau^5_{\gamma,\beta} \tau^6_{\gamma,\beta} \quad (3r_T r_V^2) \quad (1651)$$

$$\tau^8_{\gamma,\alpha} = \sum_{\delta \in A} Z_{\gamma,\delta} \tau^7_{\delta,\alpha} \quad (2r_T^2 r_V) \quad (1652)$$

$$\tau^8_{\gamma,\alpha} = \sum_{\delta \in A} Z_{\delta,\gamma} \tau^7_{\delta,\alpha} \quad (2r_T^2 r_V) \quad (1665)$$

$$\tau^9_{\gamma,\delta,w} = \sum_{\alpha \in B} \tau^8_{\gamma,\alpha} \tau^2_{\delta,\alpha,w} \tau^4_{\delta,\alpha,w} \quad (3r_D r_T^2 r_V) \quad (1653)$$

$$\tau^9_{\gamma,\delta,w} = \sum_{\alpha \in B} \tau^8_{\gamma,\alpha} \tau^2_{\delta,\alpha,w} \tau^4_{\delta,\alpha,w} \quad (3r_D r_T^2 r_V) \quad (1666)$$

$$\tau^{10}_{\gamma,\delta,w} = \sum_{\epsilon \in A} Z^*_{\delta,\epsilon} \tau^9_{\gamma,\epsilon,w} \quad (2r_D r_T^3) \quad (1654)$$

$$\tau^{10}_{\gamma,\delta,w} = \sum_{\epsilon \in A} Z^*_{\delta,\epsilon} \tau^9_{\gamma,\epsilon,w} \quad (2r_D r_T^3) \quad (1667)$$

$${}^{21}R_{a,\gamma} \leftarrow - \sum_{\delta \in A} \sum_{w \in D} {}^2D^1_{a,w} Y^1_{a,\delta} \tau^0_{\delta,\gamma,w} \tau^{10}_{\delta,\gamma,w} \quad (4r_D r_T^2 N_v) \quad (1655)$$

$${}^{21}R_{a,\gamma} \leftarrow - \sum_{\delta \in A} \sum_{w \in D} {}^2D^1_{a,w} Y^3_{a,\delta} \tau^0_{\delta,\gamma,w} \tau^{10}_{\delta,\gamma,w} \quad (4r_D r_T^2 N_v) \quad (1668)$$

Raw expression

Raw expression

$${}^{21}R_{a,\epsilon} \leftarrow \sum_{\gamma \in A} \sum_{i \in O} \sum_{j \in O} \sum_{k \in O} \sum_{l \in O} \sum_{b \in V} \sum_{c \in V} \sum_{d \in V} \frac{1}{2} \quad (1656)$$

$$\begin{aligned} & {}^1T_{a,k} \quad {}^1T_{c,i} \quad Y^{2,*}_{i,\epsilon} \quad Z^*_{\epsilon,\gamma} \quad Y^{3,*}_{b,\gamma} \\ & Y^{4,*}_{j,\gamma} \quad {}^2D^{a,i,b,j} \quad {}^2T_{d,l,b,j} \quad V_{k,d,l,c} \end{aligned}$$

$${}^{21}R_{a,\epsilon} \leftarrow \sum_{\gamma \in A} \sum_{i \in O} \sum_{j \in O} \sum_{k \in O} \sum_{l \in O} \sum_{b \in V} \sum_{c \in V} \sum_{d \in V} \frac{1}{2} \quad (1669)$$

$$\begin{aligned} & {}^1T_{a,k} \quad {}^1T_{c,j} \quad Y^{2,*}_{i,\epsilon} \quad Z^*_{\epsilon,\gamma} \quad Y^{3,*}_{b,\gamma} \\ & Y^{4,*}_{j,\gamma} \quad {}^2D^{a,i,b,j} \quad {}^2T_{b,l,d,i} \quad V_{k,d,l,c} \end{aligned}$$

Factorized expression

Factorized expression

$$\tau^0_{\gamma,\delta,w} = \sum_{i \in O} {}^2D^2_{i,w} Y^4_{i,\gamma} Y^{2,*}_{i,\delta} \quad (3r_D r_T^2 N_o) \quad (1657)$$

$$\tau^0_{\gamma,\delta,w} = \sum_{i \in O} {}^2D^2_{i,w} Y^2_{i,\gamma} Y^{2,*}_{i,\delta} \quad (3r_D r_T^2 N_o) \quad (1670)$$

$$\tau^1_{\alpha,i} = \sum_{a \in V} {}^1T_{a,i} W^2_{a,\alpha} \quad (2r_V N_o N_v) \quad (1658)$$

$$\tau^1_{\gamma,\delta,w} = \sum_{i \in O} {}^2D^4_{i,w} Y^4_{i,\gamma} Y^{4,*}_{i,\delta} \quad (3r_D r_T^2 N_o) \quad (1671)$$

$$\tau^2_{\gamma,\alpha,w} = \sum_{i \in O} {}^2D^4_{i,w} Y^{4,*}_{i,\gamma} \tau^1_{\alpha,i} \quad (3r_D r_T r_V N_o) \quad (1659)$$

$$\tau^2_{\gamma,w,i} = \sum_{a \in V} {}^2D^3_{a,w} {}^1T_{a,i} Y^{3,*}_{a,\gamma} \quad (3r_D r_T N_o N_v) \quad (1672)$$

$$\tau^3_{\gamma,w,i} = \sum_{a \in V} {}^2D^3_{a,w} {}^1T_{a,i} Y^{3,*}_{a,\gamma} \quad (3r_D r_T N_o N_v) \quad (1660)$$

$$\tau^3_{\alpha,i} = \sum_{a \in V} {}^1T_{a,i} W^4_{a,\alpha} \quad (2r_V N_o N_v) \quad (1673)$$

$$\tau^4_{\gamma,\alpha,w} = \sum_{i \in O} W^1_{i,\alpha} \tau^3_{\gamma,w,i} \quad (2r_D r_T r_V N_o) \quad (1661)$$

$$\tau^4_{\alpha} = \sum_{i \in O} W^3_{i,\alpha} \tau^3_{\alpha,i} \quad (2r_V N_o) \quad (1674)$$

$$\tau^5_{\gamma,\alpha} = \sum_{a \in V} W^4_{a,\alpha} Y^1_{a,\gamma} \quad (2r_T r_V N_v) \quad (1662)$$

$$\tau^5_{\alpha} = \sum_{\beta \in B} \tau^4_{\beta} X_{\alpha,\beta} \quad (2r_V^2) \quad (1675)$$

$$\tau^6_{\gamma,\alpha} = \sum_{i \in O} W^3_{i,\alpha} Y^2_{i,\gamma} \quad (2r_T r_V N_o) \quad (1663)$$

$$\tau^6_{i,a} = \sum_{\alpha \in B} \tau^5_{\alpha} W^1_{i,\alpha} W^2_{a,\alpha} \quad (3r_V N_o N_v) \quad (1676)$$

$$\tau^7_{\gamma,\alpha} = \sum_{\beta \in B} X_{\alpha,\beta} \tau^5_{\gamma,\beta} \tau^6_{\gamma,\beta} \quad (3r_T r_V^2) \quad (1664)$$

$$\tau^7_{\gamma,i} = \sum_{a \in V} Y^3_{a,\gamma} \tau^6_{i,a} \quad (2r_T N_o N_v) \quad (1677)$$

$$\tau^8_{\gamma,\delta,w} = \sum_{i \in O} \tau^7_{\gamma,i} \tau^2_{\delta,w,i} \quad (2r_D r_T^2 N_o) \quad (1678)$$

$$\tau^8_{\gamma,\delta,w} = \sum_{i \in O} \tau^7_{\gamma,i} \tau^2_{\delta,w,i} \quad (2r_D r_T^2 N_o) \quad (1691)$$

$$\tau^9_{\gamma,\delta,w} = \sum_{\epsilon \in A} Z^*_{\delta,\epsilon} \tau^1_{\gamma,\epsilon,w} \tau^8_{\gamma,\epsilon,w} \quad (3r_D r_T^3) \quad (1679)$$

$$\tau^9_{\gamma,\delta,w} = \sum_{\epsilon \in A} Z^*_{\delta,\epsilon} \tau^1_{\gamma,\epsilon,w} \tau^8_{\gamma,\epsilon,w} \quad (3r_D r_T^3) \quad (1692)$$

$$\tau^{10}_{\gamma,\delta,w} = \sum_{\epsilon \in A} Z_{\gamma,\epsilon} \tau^9_{\epsilon,\delta,w} \quad (2r_D r_T^3) \quad (1680)$$

$$\tau^{10}_{\gamma,\delta,w} = \sum_{\epsilon \in A} Z_{\epsilon,\gamma} \tau^9_{\epsilon,\delta,w} \quad (2r_D r_T^3) \quad (1693)$$

$${}^{21}R_{a,\gamma} \leftarrow - \sum_{\delta \in A} \sum_{w \in D} {}^2D^1_{a,w} Y^1_{a,\delta} \tau^0_{\delta,\gamma,w} \tau^{10}_{\delta,\gamma,w} \quad (4r_D r_T^2 N_v) \quad (1681)$$

$$R_{a,\gamma} \leftarrow - \sum_{\delta \in A} \sum_{w \in D} {}^2D^1_{a,w} Y^3_{a,\delta} \tau^0_{\delta,\gamma,w} \tau^{10}_{\delta,\gamma,w} \quad (4r_D r_T^2 N_v) \quad (1694)$$

Raw expression

Raw expression

$${}^{21}R_{a,\epsilon} \leftarrow \sum_{\gamma \in A} \sum_{i \in O} \sum_{j \in O} \sum_{k \in O} \sum_{l \in O} \sum_{b \in V} \sum_{c \in V} \sum_{d \in V} \frac{1}{2} \quad (1682)$$

$$\begin{matrix} {}^1T_{a,k} & {}^1T_{c,j} & Y^{2,*}_{i,\epsilon} & Z^*_{\epsilon,\gamma} & Y^{3,*}_{b,\gamma} \\ Y^{4,*}_{j,\gamma} & {}^2D^{a,i,b,j} & {}^2T_{d,i,b,l} & V_{k,d,l,c} \end{matrix}$$

$${}^{21}R_{a,\epsilon} \leftarrow \sum_{\gamma \in A} \sum_{i \in O} \sum_{j \in O} \sum_{k \in O} \sum_{l \in O} \sum_{b \in V} \sum_{c \in V} \sum_{d \in V} \frac{1}{2} \quad (1695)$$

$$\begin{matrix} {}^1T_{a,k} & {}^1T_{c,l} & Y^{2,*}_{i,\epsilon} & Z^*_{\epsilon,\gamma} & Y^{3,*}_{b,\gamma} \\ Y^{4,*}_{j,\gamma} & {}^2D^{a,i,b,j} & {}^2T_{b,j,d,i} & V_{k,c,l,d} \end{matrix}$$

Factorized expression

Factorized expression

$$\tau^0_{\gamma,\delta,w} = \sum_{i \in O} {}^2D^2_{i,w} Y^4_{i,\gamma} Y^{2,*}_{i,\delta} \quad (3r_D r_T^2 N_o) \quad (1683)$$

$$\tau^0_{\gamma,\delta,w} = \sum_{a \in V} {}^2D^3_{a,w} Y^1_{a,\gamma} Y^{3,*}_{a,\delta} \quad (3r_D r_T^2 N_v) \quad (1696)$$

$$\tau^1_{\gamma,\delta,w} = \sum_{i \in O} {}^2D^4_{i,w} Y^2_{i,\gamma} Y^{4,*}_{i,\delta} \quad (3r_D r_T^2 N_o) \quad (1684)$$

$$\tau^1_{\gamma,\delta,w} = \sum_{i \in O} {}^2D^4_{i,w} Y^2_{i,\gamma} Y^{4,*}_{i,\delta} \quad (3r_D r_T^2 N_o) \quad (1697)$$

$$\tau^2_{\gamma,w,i} = \sum_{a \in V} {}^2D^3_{a,w} {}^1T_{a,i} Y^{3,*}_{a,\gamma} \quad (3r_D r_T N_o N_v) \quad (1685)$$

$$\tau^2_{\gamma,\delta,w} = \sum_{\epsilon \in A} Z^*_{\delta,\epsilon} \tau^0_{\gamma,\epsilon,w} \tau^1_{\gamma,\epsilon,w} \quad (3r_D r_T^3) \quad (1698)$$

$$\tau^3_{\alpha,i} = \sum_{a \in V} {}^1T_{a,i} W^4_{a,\alpha} \quad (2r_V N_o N_v) \quad (1686)$$

$$\tau^3_{\gamma,\delta,w} = \sum_{\epsilon \in A} Z_{\epsilon,\gamma} \tau^2_{\epsilon,\delta,w} \quad (2r_D r_T^3) \quad (1699)$$

$$\tau^4_{\alpha} = \sum_{i \in O} W^3_{i,\alpha} \tau^3_{\alpha,i} \quad (2r_V N_o) \quad (1687)$$

$$\tau^4_{\alpha,i} = \sum_{a \in V} {}^1T_{a,i} W^2_{a,\alpha} \quad (2r_V N_o N_v) \quad (1700)$$

$$\tau^5_{\alpha} = \sum_{\beta \in B} \tau^4_{\beta} X_{\alpha,\beta} \quad (2r_V^2) \quad (1688)$$

$$\tau^5_{\alpha} = \sum_{i \in O} W^1_{i,\alpha} \tau^4_{\alpha,i} \quad (2r_V N_o) \quad (1701)$$

$$\tau^6_{i,a} = \sum_{\alpha \in B} \tau^5_{\alpha} W^1_{i,\alpha} W^2_{a,\alpha} \quad (3r_V N_o N_v) \quad (1689)$$

$$\tau^6_{\alpha} = \sum_{\beta \in B} \tau^5_{\beta} X_{\beta,\alpha} \quad (2r_V^2) \quad (1702)$$

$$\tau^7_{\gamma,i} = \sum_{a \in V} Y^1_{a,\gamma} \tau^6_{i,a} \quad (2r_T N_o N_v) \quad (1690)$$

$$\tau^7_{i,a} = \sum_{\alpha \in B} \tau^6_{\alpha} W^3_{i,\alpha} W^4_{a,\alpha} \quad (3r_V N_o N_v) \quad (1703)$$

$$\tau_{i,j}^8 = \sum_{a \in V} {}^1T_{a,i} \tau_{j,a}^7 \quad (2N_o^2 N_v) \quad (1704)$$

$$\tau_{\gamma,\delta,w}^8 = \sum_{i \in O} {}^2D_{i,w}^4 Y_{i,\delta}^{4,*} \tau_{\gamma,i}^7 \quad (3r_D r_T^2 N_o) \quad (1717)$$

$$\tau_{\gamma,i}^9 = \sum_{j \in O} Y_{j,\gamma}^4 \tau_{i,j}^8 \quad (2r_T N_o^2) \quad (1705)$$

$$\tau_{\gamma,\delta,w}^9 = \sum_{\epsilon \in A} Z_{\delta,\epsilon}^* \tau_{\gamma,\epsilon,w}^1 \tau_{\gamma,\epsilon,w}^8 \quad (3r_D r_T^3) \quad (1718)$$

$$\tau_{\gamma,\delta,w}^{10} = \sum_{i \in O} {}^2D_{i,w}^2 Y_{i,\delta}^{2,*} \tau_{\gamma,i}^9 \quad (3r_D r_T^2 N_o) \quad (1706)$$

$$\tau_{\gamma,\delta,w}^{10} = \sum_{\epsilon \in A} Z_{\epsilon,\gamma} \tau_{\epsilon,\delta,w}^9 \quad (2r_D r_T^3) \quad (1719)$$

$${}^{21}R_{a,\gamma} \leftarrow - \sum_{\delta \in A} \sum_{w \in D} {}^2D_{a,w}^1 Y_{a,\delta}^3 \tau_{\delta,\gamma,w}^{10} \tau_{\delta,\gamma,w}^3 \quad (4r_D r_T^2 N_v) \quad (1707)$$

$${}^{21}R_{a,\gamma} \leftarrow - \sum_{\delta \in A} \sum_{w \in D} {}^2D_{a,w}^1 Y_{a,\delta}^3 \tau_{\delta,\gamma,w}^0 \tau_{\delta,\gamma,w}^{10} \quad (4r_D r_T^2 N_v) \quad (1720)$$

Raw expression

Raw expression

$${}^{21}R_{a,\epsilon} \leftarrow \sum_{\gamma \in A} \sum_{i \in O} \sum_{j \in O} \sum_{k \in O} \sum_{l \in O} \sum_{b \in V} \sum_{c \in V} \sum_{d \in V} \frac{1}{2} \quad (1708)$$

$${}^1T_{a,k} {}^1T_{c,l} Y_{i,\epsilon}^{2,*} Z_{\epsilon,\gamma}^* Y_{b,\gamma}^{3,*} Y_{j,\gamma}^{4,*} {}^2D_{a,i,b,j} {}^2T_{d,i,b,j} V_{k,c,l,d}$$

$${}^{21}R_{a,\epsilon} \leftarrow \sum_{\gamma \in A} \sum_{i \in O} \sum_{j \in O} \sum_{k \in O} \sum_{l \in O} \sum_{b \in V} \sum_{c \in V} \sum_{d \in V} \frac{1}{2} \quad (1721)$$

$${}^1T_{b,k} {}^1T_{c,i} Y_{i,\epsilon}^{2,*} Z_{\epsilon,\gamma}^* Y_{b,\gamma}^{3,*} Y_{j,\gamma}^{4,*} {}^2D_{a,i,b,j} {}^2T_{a,l,d,j} V_{k,d,l,c}$$

Factorized expression

Factorized expression

$$\tau_{\gamma,\delta,w}^0 = \sum_{i \in O} {}^2D_{i,w}^2 Y_{i,\gamma}^4 Y_{i,\delta}^{2,*} \quad (3r_D r_T^2 N_o) \quad (1709)$$

$$\tau_{\gamma,\delta,w}^0 = \sum_{a \in V} {}^2D_{a,w}^3 Y_{a,\gamma}^3 Y_{a,\delta}^{3,*} \quad (3r_D r_T^2 N_v) \quad (1722)$$

$$\tau_{\gamma,\delta,w}^1 = \sum_{a \in V} {}^2D_{a,w}^3 Y_{a,\gamma}^1 Y_{a,\delta}^{3,*} \quad (3r_D r_T^2 N_v) \quad (1710)$$

$$\tau_{\gamma,\delta,w}^1 = \sum_{i \in O} {}^2D_{i,w}^4 Y_{i,\gamma}^4 Y_{i,\delta}^{4,*} \quad (3r_D r_T^2 N_o) \quad (1723)$$

$$\tau_{\alpha,i}^2 = \sum_{a \in V} {}^1T_{a,i} W_{a,\alpha}^2 \quad (2r_V N_o N_v) \quad (1711)$$

$$\tau_{\gamma,\delta,w}^2 = \sum_{\epsilon \in A} Z_{\delta,\epsilon}^* \tau_{\gamma,\epsilon,w}^0 \tau_{\gamma,\epsilon,w}^1 \quad (3r_D r_T^3) \quad (1724)$$

$$\tau_{\alpha}^3 = \sum_{i \in O} W_{i,\alpha}^1 \tau_{\alpha,i}^2 \quad (2r_V N_o) \quad (1712)$$

$$\tau_{\gamma,\delta,w}^3 = \sum_{\epsilon \in A} Z_{\gamma,\epsilon} \tau_{\epsilon,\delta,w}^2 \quad (2r_D r_T^3) \quad (1725)$$

$$\tau_{\alpha}^4 = \sum_{\beta \in B} \tau_{\beta}^3 X_{\beta,\alpha} \quad (2r_V^2) \quad (1713)$$

$$\tau_{\alpha,i}^4 = \sum_{a \in V} {}^1T_{a,i} W_{a,\alpha}^2 \quad (2r_V N_o N_v) \quad (1726)$$

$$\tau_{i,a}^5 = \sum_{\alpha \in B} \tau_{\alpha}^4 W_{i,\alpha}^3 W_{a,\alpha}^4 \quad (3r_V N_o N_v) \quad (1714)$$

$$\tau_{\alpha}^5 = \sum_{i \in O} W_{i,\alpha}^1 \tau_{\alpha,i}^4 \quad (2r_V N_o) \quad (1727)$$

$$\tau_{i,j}^6 = \sum_{a \in V} {}^1T_{a,i} \tau_{j,a}^5 \quad (2N_o^2 N_v) \quad (1715)$$

$$\tau_{\alpha}^6 = \sum_{\beta \in B} \tau_{\beta}^5 X_{\beta,\alpha} \quad (2r_V^2) \quad (1728)$$

$$\tau_{\gamma,i}^7 = \sum_{j \in O} Y_{j,\gamma}^2 \tau_{i,j}^6 \quad (2r_T N_o^2) \quad (1716)$$

$$\tau_{i,a}^7 = \sum_{\alpha \in B} \tau_{\alpha}^6 W_{i,\alpha}^3 W_{a,\alpha}^4 \quad (3r_V N_o N_v) \quad (1729)$$

$$\tau^8_{i,j} = \sum_{a \in V} {}^1T_{a,i} \tau^7_{j,a} \quad (2N_o^2 N_v) \quad (1730)$$

$$\tau^8_{\gamma,\delta,w} = \sum_{i \in O} {}^2D^4_{i,w} Y^{4,*}_{i,\delta} \tau^7_{\gamma,i} \quad (3r_D r_T^2 N_o) \quad (1743)$$

$$\tau^9_{\gamma,i} = \sum_{j \in O} Y^2_{j,\gamma} \tau^8_{i,j} \quad (2r_T N_o^2) \quad (1731)$$

$$\tau^9_{\gamma,\delta,w} = \sum_{\epsilon \in A} Z^*_{\delta,\epsilon} \tau^1_{\gamma,\epsilon,w} \tau^8_{\gamma,\epsilon,w} \quad (3r_D r_T^3) \quad (1744)$$

$$\tau^{10}_{\gamma,\delta,w} = \sum_{i \in O} {}^2D^2_{i,w} Y^{2,*}_{i,\delta} \tau^9_{\gamma,i} \quad (3r_D r_T^2 N_o) \quad (1732)$$

$$\tau^{10}_{\gamma,\delta,w} = \sum_{\epsilon \in A} Z_{\gamma,\epsilon} \tau^9_{\epsilon,\delta,w} \quad (2r_D r_T^3) \quad (1745)$$

$${}^{21}R_{a,\gamma} \leftarrow - \sum_{\delta \in A} \sum_{w \in D} {}^2D^1_{a,w} Y^1_{a,\delta} \tau^{10}_{\delta,\gamma,w} \tau^3_{\delta,\gamma,w} \quad (4r_D r_T^2 N_o) \quad (1733)$$

$${}^{21}R_{a,\gamma} \leftarrow - \sum_{\delta \in A} \sum_{w \in D} {}^2D^1_{a,w} Y^1_{a,\delta} \tau^0_{\delta,\gamma,w} \tau^{10}_{\delta,\gamma,w} \quad (4r_D r_T^2 N_v) \quad (1746)$$

Raw expression

$${}^{21}R_{a,\epsilon} \leftarrow \sum_{\gamma \in A} \sum_{i \in O} \sum_{j \in O} \sum_{k \in O} \sum_{l \in O} \sum_{b \in V} \sum_{c \in V} \sum_{d \in V} \frac{1}{2} \quad (1734)$$

$${}^1T_{b,k} {}^1T_{c,i} Y^{2,*}_{i,\epsilon} Z^*_{\epsilon,\gamma} Y^{3,*}_{b,\gamma} Y^{4,*}_{j,\gamma} {}^2D^{a,i,b,j} {}^2T_{d,j,a,l} V_{k,d,l,c}$$

Raw expression

$${}^{21}R_{a,\epsilon} \leftarrow \sum_{\gamma \in A} \sum_{i \in O} \sum_{j \in O} \sum_{k \in O} \sum_{l \in O} \sum_{b \in V} \sum_{c \in V} \sum_{d \in V} \frac{1}{2} \quad (1747)$$

$${}^1T_{b,k} {}^1T_{c,j} Y^{2,*}_{i,\epsilon} Z^*_{\epsilon,\gamma} Y^{3,*}_{b,\gamma} Y^{4,*}_{j,\gamma} {}^2D^{a,i,b,j} {}^2T_{a,i,d,l} V_{k,d,l,c}$$

Factorized expression

$$\tau^0_{\gamma,\delta,w} = \sum_{i \in O} {}^2D^2_{i,w} Y^2_{i,\gamma} Y^{2,*}_{i,\delta} \quad (3r_D r_T^2 N_o) \quad (1735)$$

$$\tau^0_{\gamma,w,i} = \sum_{a \in V} {}^2D^3_{a,w} {}^1T_{a,i} Y^{3,*}_{a,\gamma} \quad (3r_D r_T N_o N_v) \quad (1748)$$

$$\tau^1_{\gamma,\delta,w} = \sum_{a \in V} {}^2D^3_{a,w} Y^3_{a,\gamma} Y^{3,*}_{a,\delta} \quad (3r_D r_T^2 N_v) \quad (1736)$$

$$\tau^1_{\gamma,\alpha} = \sum_{a \in V} W^2_{a,\alpha} Y^1_{a,\gamma} \quad (2r_T r_V N_v) \quad (1749)$$

$$\tau^2_{\alpha,i} = \sum_{a \in V} {}^1T_{a,i} W^2_{a,\alpha} \quad (2r_V N_o N_v) \quad (1737)$$

$$\tau^2_{\gamma,\alpha,i} = \sum_{\beta \in B} W^1_{i,\beta} X_{\beta,\alpha} \tau^1_{\gamma,\beta} \quad (3r_T r_V^2 N_o) \quad (1750)$$

$$\tau^3_{\alpha} = \sum_{i \in O} W^1_{i,\alpha} \tau^2_{\alpha,i} \quad (2r_V N_o) \quad (1738)$$

$$\tau^3_{\gamma,\alpha} = \sum_{a \in V} W^4_{a,\alpha} Y^3_{a,\gamma} \quad (2r_T r_V N_v) \quad (1751)$$

$$\tau^4_{\alpha} = \sum_{\beta \in B} \tau^3_{\beta} X_{\beta,\alpha} \quad (2r_V^2) \quad (1739)$$

$$\tau^4_{\gamma,\alpha,i} = \sum_{\delta \in A} Z_{\gamma,\delta} Y^4_{i,\delta} \tau^3_{\delta,\alpha} \quad (3r_T^2 r_V N_o) \quad (1752)$$

$$\tau^5_{i,a} = \sum_{\alpha \in B} \tau^4_{\alpha} W^3_{i,\alpha} W^4_{a,\alpha} \quad (3r_V N_o N_v) \quad (1740)$$

$$\tau^5_{\gamma,i,j,k} = \sum_{\alpha \in B} W^3_{j,\alpha} \tau^2_{\gamma,\alpha,i} \tau^4_{\gamma,\alpha,k} \quad (3r_T r_V N_o^3) \quad (1753)$$

$$\tau^6_{i,j} = \sum_{a \in V} {}^1T_{a,i} \tau^5_{j,a} \quad (2N_o^2 N_v) \quad (1741)$$

$$\tau^7_{\gamma,i} = \sum_{j \in O} Y^4_{j,\gamma} \tau^6_{i,j} \quad (2r_T N_o^2) \quad (1742)$$

$$\tau^6_{i,j,k,l} = \sum_{\gamma \in A} Y^2_{k,\gamma} \tau^5_{\gamma,i,j,l} \quad (2r_T N_o^4) \quad (1754)$$

$$\tau_{\gamma,w,i,j}^7 = \sum_{k \in O} \sum_{l \in O} {}^2D_{k,w}^4 Y_{k,\gamma}^{4,*} \tau_{\gamma,w,l}^0 \tau_{i,l,j,k}^6 \quad (4r_D r_T N_o^4) \tau_{\gamma,w,i}^8 = \sum_{\delta \in A} \sum_{j \in O} {}^2D_{j,w}^2 Y_{j,\gamma}^{2,*} Z_{\gamma,\delta}^* \tau_{\delta,w,i,j}^7 \quad (4r_D r_T^2 N_o^2) \quad (1755) \quad (1767)$$

$$\tau_{\gamma,w,i}^8 = \sum_{\delta \in A} \sum_{j \in O} {}^2D_{j,w}^2 Y_{j,\gamma}^{2,*} Z_{\gamma,\delta}^* \tau_{\delta,w,i,j}^7 \quad (4r_D r_T^2 N_o^2) \quad {}^{21}R_{a,\gamma} \leftarrow \sum_{w \in D} \sum_{i \in O} \frac{1}{2} {}^2D_{a,w}^1 {}^1T_{a,i} {}^8\tau_{\gamma,w,i} \quad (3r_D r_T N_o N_v) \quad (1756) \quad (1768)$$

$${}^{21}R_{a,\gamma} \leftarrow \sum_{w \in D} \sum_{i \in O} \frac{1}{2} {}^2D_{a,w}^1 {}^1T_{a,i} {}^8\tau_{\gamma,w,i} \quad (3r_D r_T N_o N_v) \quad (1757)$$

Raw expression

$${}^{21}R_{a,\epsilon} \leftarrow \sum_{\gamma \in A} \sum_{i \in O} \sum_{j \in O} \sum_{k \in O} \sum_{l \in O} \sum_{b \in V} \sum_{c \in V} \sum_{d \in V} \frac{1}{2} {}^1T_{b,k} {}^1T_{c,j} Y_{i,\epsilon}^{2,*} Z_{\epsilon,\gamma}^* Y_{b,\gamma}^{3,*} Y_{j,\gamma}^{4,*} {}^2D_{a,i,b,j} {}^2T_{a,l,d,i} V_{k,c,l,d} \quad (1758)$$

Raw expression

$${}^{21}R_{a,\epsilon} \leftarrow \sum_{\gamma \in A} \sum_{i \in O} \sum_{j \in O} \sum_{k \in O} \sum_{l \in O} \sum_{b \in V} \sum_{c \in V} \sum_{d \in V} \frac{1}{2} {}^1T_{b,k} {}^1T_{c,j} Y_{i,\epsilon}^{2,*} Z_{\epsilon,\gamma}^* Y_{b,\gamma}^{3,*} Y_{j,\gamma}^{4,*} {}^2D_{a,i,b,j} {}^2T_{d,i,a,l} V_{k,c,l,d} \quad (1769)$$

Factorized expression

$$\tau_{\gamma,\delta,w}^0 = \sum_{a \in V} {}^2D_{a,w}^3 Y_{a,\gamma}^1 Y_{a,\delta}^{3,*} \quad (3r_D r_T^2 N_v) \quad (1770)$$

Factorized expression

$$\tau_{\gamma,w,i}^0 = \sum_{a \in V} {}^2D_{a,w}^3 {}^1T_{a,i} Y_{a,\gamma}^{3,*} \quad (3r_D r_T N_o N_v) \quad (1759)$$

$$\tau_{\gamma,\alpha}^1 = \sum_{i \in O} W_{i,\alpha}^3 Y_{i,\gamma}^2 \quad (2r_T r_V N_o) \quad (1771)$$

$$\tau_{\gamma,\alpha}^1 = \sum_{a \in V} W_{a,\alpha}^4 Y_{a,\gamma}^1 \quad (2r_T r_V N_v) \quad (1760)$$

$$\tau_{\gamma,\alpha}^2 = \sum_{a \in V} W_{a,\alpha}^4 Y_{a,\gamma}^3 \quad (2r_T r_V N_v) \quad (1772)$$

$$\tau_{\gamma,\alpha,i}^2 = \sum_{\beta \in B} X_{\alpha,\beta} W_{i,\beta}^3 \tau_{\gamma,\beta}^1 \quad (3r_T r_V^2 N_o) \quad (1761)$$

$$\tau_{\gamma,\alpha,i}^3 = \sum_{\delta \in A} Z_{\gamma,\delta} Y_{i,\delta}^4 \tau_{\delta,\alpha}^2 \quad (3r_T^2 r_V N_o) \quad (1773)$$

$$\tau_{\gamma,\alpha}^3 = \sum_{a \in V} W_{a,\alpha}^2 Y_{a,\gamma}^3 \quad (2r_T r_V N_v) \quad (1762)$$

$$\tau_{\gamma,\alpha,w}^4 = \sum_{\delta \in A} \sum_{i \in O} {}^2D_{i,w}^4 Y_{i,\gamma}^{4,*} \tau_{\delta,\alpha}^1 \tau_{\delta,\gamma,w}^0 \tau_{\delta,\alpha,i}^3 \quad (5r_D r_T^2 r_V N_o) \quad (1774)$$

$$\tau_{\gamma,\alpha,i}^4 = \sum_{\delta \in A} Z_{\gamma,\delta} Y_{i,\delta}^4 \tau_{\delta,\alpha}^3 \quad (3r_T^2 r_V N_o) \quad (1763)$$

$$\tau_{\gamma,\alpha,w}^5 = \sum_{\beta \in B} X_{\alpha,\beta} \tau_{\gamma,\beta,w}^4 \quad (2r_D r_T r_V^2) \quad (1775)$$

$$\tau_{\gamma,i,j,k}^5 = \sum_{\alpha \in B} W_{i,\alpha}^1 \tau_{\gamma,\alpha,j}^2 \tau_{\gamma,\alpha,k}^4 \quad (3r_T r_V N_o^3) \quad (1764)$$

$$\tau_{\gamma,\alpha,w}^6 = \sum_{\delta \in A} Z_{\gamma,\delta}^* \tau_{\delta,\alpha,w}^5 \quad (2r_D r_T^2 r_V) \quad (1776)$$

$$\tau_{i,j,k,l}^6 = \sum_{\gamma \in A} Y_{k,\gamma}^2 \tau_{\gamma,i,j,l}^5 \quad (2r_T N_o^4) \quad (1765)$$

$$\tau_{\alpha,i}^7 = \sum_{a \in V} {}^1T_{a,i} W_{a,\alpha}^2 \quad (2r_V N_o N_v) \quad (1777)$$

$$\tau_{\gamma,w,i,j}^7 = \sum_{k \in O} \sum_{l \in O} {}^2D_{k,w}^4 Y_{k,\gamma}^{4,*} \tau_{\gamma,w,l}^0 \tau_{i,l,k,j}^6 \quad (4r_D r_T N_o^4) \quad \tau_{\gamma,\alpha,w}^8 = \sum_{i \in O} {}^2D_{i,w}^2 Y_{i,\gamma}^{2,*} \tau_{\alpha,i}^7 \quad (3r_D r_T r_V N_o) \quad (1778) \quad (1766)$$

$$\tau_{\gamma,w,i}^9 = \sum_{\alpha \in B} W_{i,\alpha}^1 \tau_{\gamma,\alpha,w}^6 \tau_{\gamma,\alpha,w}^8 \quad (3r_D r_T r_V N_o) \quad (1779)$$

$$\tau_{\gamma,w,i}^9 = \sum_{\alpha \in B} W_{i,\alpha}^1 \tau_{\gamma,\alpha,w}^6 \tau_{\gamma,\alpha,w}^8 \quad (3r_D r_T r_V N_o) \quad (1791)$$

$${}^{21}R_{a,\gamma} \leftarrow \sum_{w \in D} \sum_{i \in O} \frac{1}{2} D_{a,w}^1 T_{a,i}^1 \tau_{\gamma,w,i}^9 \quad (3r_D r_T N_o N_v) \quad (1780)$$

$${}^{21}R_{a,\gamma} \leftarrow \sum_{w \in D} \sum_{i \in O} \frac{1}{2} D_{a,w}^1 T_{a,i}^1 \tau_{\gamma,w,i}^9 \quad (3r_D r_T N_o N_v) \quad (1792)$$

Raw expression

$${}^{21}R_{a,\epsilon} \leftarrow \sum_{\gamma \in A} \sum_{i \in O} \sum_{j \in O} \sum_{k \in O} \sum_{l \in O} \sum_{b \in V} \sum_{c \in V} \sum_{d \in V} \frac{1}{2} \quad (1781)$$

$${}^1T_{b,k} {}^1T_{c,j} Y_{i,\epsilon}^{2,*} Z_{\epsilon,\gamma}^* Y_{b,\gamma}^{3,*} Y_{j,\gamma}^{4,*} {}^2D_{a,i,b,j} {}^2T_{d,l,a,i} V_{k,d,l,c}$$

Raw expression

$${}^{21}R_{a,\epsilon} \leftarrow \sum_{\gamma \in A} \sum_{i \in O} \sum_{j \in O} \sum_{k \in O} \sum_{l \in O} \sum_{b \in V} \sum_{c \in V} \sum_{d \in V} \frac{1}{2} \quad (1793)$$

$${}^1T_{b,k} {}^1T_{c,l} Y_{i,\epsilon}^{2,*} Z_{\epsilon,\gamma}^* Y_{b,\gamma}^{3,*} Y_{j,\gamma}^{4,*} {}^2D_{a,i,b,j} {}^2T_{a,i,d,j} V_{k,c,l,d}$$

Factorized expression

$$\tau_{\gamma,\delta,w}^0 = \sum_{a \in V} {}^2D_{a,w}^3 Y_{a,\gamma}^3 Y_{a,\delta}^{3,*} \quad (3r_D r_T^2 N_v) \quad (1782)$$

$$\tau_{\gamma,\alpha}^0 = \sum_{a \in V} W_{a,\alpha}^2 Y_{a,\gamma}^3 \quad (2r_T r_V N_v) \quad (1794)$$

$$\tau_{\gamma,\alpha}^1 = \sum_{a \in V} W_{a,\alpha}^4 Y_{a,\gamma}^1 \quad (2r_T r_V N_v) \quad (1783)$$

$$\tau_{\alpha,i}^1 = \sum_{a \in V} {}^1T_{a,i} W_{a,\alpha}^4 \quad (2r_V N_o N_v) \quad (1795)$$

$$\tau_{\gamma,\alpha,i}^2 = \sum_{\delta \in A} Y_{i,\delta}^2 Z_{\delta,\gamma} \tau_{\delta,\alpha}^1 \quad (3r_T^2 r_V N_o) \quad (1784)$$

$$\tau_{\alpha,i,j}^2 = \sum_{\beta \in B} X_{\alpha,\beta} W_{j,\beta}^3 \tau_{\beta,i}^1 \quad (3r_V^2 N_o^2) \quad (1796)$$

$$\tau_{\gamma,\alpha}^3 = \sum_{i \in O} W_{i,\alpha}^3 Y_{i,\gamma}^4 \quad (2r_T r_V N_o) \quad (1785)$$

$$\tau_{\gamma,\alpha,i}^3 = \sum_{j \in O} Y_{j,\gamma}^4 \tau_{\alpha,i,j}^2 \quad (2r_T r_V N_o^2) \quad (1797)$$

$$\tau_{\gamma,\alpha,w}^4 = \sum_{\delta \in A} \sum_{i \in O} {}^2D_{i,w}^4 Y_{i,\gamma}^{4,*} \tau_{i,\gamma}^3 \tau_{\delta,\alpha}^0 \tau_{\delta,\gamma,w}^0 \tau_{\delta,\alpha,i}^2 \quad (5r_D r_T^2 r_V N_o) \quad (1786)$$

$$\tau_{\gamma,i,j}^4 = \sum_{\alpha \in B} W_{j,\alpha}^1 \tau_{\gamma,\alpha}^0 \tau_{\gamma,\alpha,i}^3 \quad (3r_T r_V N_o^2) \quad (1798)$$

$$\tau_{\gamma,i,j}^5 = \sum_{\delta \in A} Z_{\gamma,\delta} \tau_{\delta,i,j}^4 \quad (2r_T^2 N_o^2) \quad (1799)$$

$$\tau_{\gamma,\alpha,w}^5 = \sum_{\beta \in B} X_{\alpha,\beta} \tau_{\gamma,\beta,w}^4 \quad (2r_D r_T r_V^2) \quad (1787)$$

$$\tau_{\gamma,\delta,w}^6 = \sum_{a \in V} {}^2D_{a,w}^3 Y_{a,\gamma}^1 Y_{a,\delta}^{3,*} \quad (3r_D r_T^2 N_v) \quad (1800)$$

$$\tau_{\gamma,\alpha,w}^6 = \sum_{\delta \in A} Z_{\gamma,\delta}^* \tau_{\delta,\alpha,w}^5 \quad (2r_D r_T^2 r_V) \quad (1788)$$

$$\tau_{\gamma,\delta,w}^7 = \sum_{i \in O} {}^2D_{i,w}^4 Y_{i,\gamma}^2 Y_{i,\delta}^{4,*} \quad (3r_D r_T^2 N_o) \quad (1801)$$

$$\tau_{\alpha,i}^7 = \sum_{a \in V} {}^1T_{a,i} W_{a,\alpha}^2 \quad (2r_V N_o N_v) \quad (1789)$$

$$\tau_{\gamma,\delta,w}^8 = \sum_{\epsilon \in A} Z_{\delta,\epsilon}^* \tau_{\gamma,\epsilon,w}^6 \tau_{\gamma,\epsilon,w}^7 \quad (3r_D r_T^3) \quad (1802)$$

$$\tau_{\gamma,\alpha,w}^8 = \sum_{i \in O} {}^2D_{i,w}^2 Y_{i,\gamma}^{2,*} \tau_{i,\gamma}^7 \tau_{\alpha,i}^7 \quad (3r_D r_T r_V N_o) \quad (1790)$$

$$\tau_{\gamma,w,i,j}^9 = \sum_{\delta \in A} \tau_{\delta,i,j}^5 \tau_{\delta,\gamma,w}^8 \quad (2r_D r_T^2 N_o^2) \quad (1803)$$



$$\tau_{\gamma,w,i}^{10} = \sum_{j \in O} {}^2D_{j,w}^2 Y_{j,\gamma}^{2,*} \tau_{\gamma,w,j,i}^9 \quad (3r_D r_T N_o^2) \quad (1804)$$

$$\tau_{\gamma,w,i}^{10} = \sum_{j \in O} {}^2D_{j,w}^2 Y_{j,\gamma}^{2,*} \tau_{\gamma,w,j,i}^9 \quad (3r_D r_T N_o^2) \quad (1817)$$

$${}^{21}R_{a,\gamma} \leftarrow \sum_{w \in D} \sum_{i \in O} \frac{1}{2} {}^2D_{a,w}^1 T_{a,i} {}^{\tau^{10}}_{\gamma,w,i} \quad (3r_D r_T N_o N_v) \quad (1805)$$

$${}^{21}R_{a,\gamma} \leftarrow \sum_{w \in D} \sum_{i \in O} \frac{1}{2} {}^2D_{a,w}^1 T_{a,i} {}^{\tau^{10}}_{\gamma,w,i} \quad (3r_D r_T N_o N_v) \quad (1818)$$

Raw expression

$${}^{21}R_{a,\epsilon} \leftarrow \sum_{\gamma \in A} \sum_{i \in O} \sum_{j \in O} \sum_{k \in O} \sum_{l \in O} \sum_{b \in V} \sum_{c \in V} \sum_{d \in V} \frac{1}{2} \quad (1806)$$

$${}^1T_{b,k} {}^1T_{c,l} Y_{i,\epsilon}^{2,*} Z_{\epsilon,\gamma}^* Y_{b,\gamma}^{3,*} Y_{j,\gamma}^{4,*} {}^2D_{a,i,b,j} {}^2T_{d,j,a,i} V_{k,c,l,d}$$

Raw expression

$${}^{21}R_{a,\epsilon} \leftarrow \sum_{\gamma \in A} \sum_{i \in O} \sum_{j \in O} \sum_{k \in O} \sum_{l \in O} \sum_{b \in V} \sum_{c \in V} \sum_{d \in V} \frac{1}{2} \quad (1819)$$

$${}^1T_{c,i} {}^1T_{d,j} Y_{i,\epsilon}^{2,*} Z_{\epsilon,\gamma}^* Y_{b,\gamma}^{3,*} Y_{j,\gamma}^{4,*} {}^2D_{a,i,b,j} {}^2T_{a,k,b,l} V_{k,c,l,d}$$

Factorized expression

$$\tau_{\gamma,\alpha}^0 = \sum_{a \in V} W_{a,\alpha}^2 Y_{a,\gamma}^1 \quad (2r_T r_V N_v) \quad (1807)$$

$$\tau_{\gamma,\alpha}^0 = \sum_{a \in V} W_{a,\alpha}^2 Y_{a,\gamma}^3 \quad (2r_T r_V N_v) \quad (1820)$$

$$\tau_{\alpha,i}^1 = \sum_{a \in V} {}^1T_{a,i} W_{a,\alpha}^4 \quad (2r_V N_o N_v) \quad (1808)$$

$$\tau_{\gamma,\alpha,i}^1 = \sum_{\delta \in A} Z_{\gamma,\delta} Y_{i,\delta}^4 \tau_{\delta,\alpha}^0 \quad (3r_T^2 r_V N_o) \quad (1821)$$

$$\tau_{\alpha,i,j}^2 = \sum_{\beta \in B} X_{\alpha,\beta} W_{j,\beta}^3 \tau_{\beta,i}^1 \quad (3r_V^2 N_o^2) \quad (1809)$$

$$\tau_{\gamma,\delta,w}^2 = \sum_{a \in V} {}^2D_{a,w}^3 Y_{a,\gamma}^1 Y_{a,\delta}^{3,*} \quad (3r_D r_T^2 N_v) \quad (1822)$$

$$\tau_{\gamma,\alpha,i}^3 = \sum_{j \in O} Y_{j,\gamma}^2 \tau_{\alpha,i,j}^2 \quad (2r_T r_V N_o^2) \quad (1810)$$

$$\tau_{\alpha,i}^3 = \sum_{a \in V} {}^1T_{a,i} W_{a,\alpha}^4 \quad (2r_V N_o N_v) \quad (1823)$$

$$\tau_{\gamma,i,j}^4 = \sum_{\alpha \in B} W_{j,\alpha}^1 \tau_{\gamma,\alpha}^0 \tau_{\gamma,\alpha,i}^3 \quad (3r_T r_V N_o^2) \quad (1811)$$

$$\tau_{\alpha,i,j}^4 = \sum_{\beta \in B} X_{\alpha,\beta} W_{j,\beta}^3 \tau_{\beta,i}^3 \quad (3r_V^2 N_o^2) \quad (1824)$$

$$\tau_{\gamma,i,j}^5 = \sum_{\delta \in A} Z_{\delta,\gamma} \tau_{\delta,i,j}^4 \quad (2r_T^2 N_o^2) \quad (1812)$$

$$\tau_{\gamma,\alpha,i}^5 = \sum_{j \in O} Y_{j,\gamma}^2 \tau_{\alpha,i,j}^4 \quad (2r_T r_V N_o^2) \quad (1825)$$

$$\tau_{\gamma,\delta,w}^6 = \sum_{a \in V} {}^2D_{a,w}^3 Y_{a,\gamma}^3 Y_{a,\delta}^{3,*} \quad (3r_D r_T^2 N_v) \quad (1813)$$

$$\tau_{\gamma,\delta,\alpha,w}^6 = \sum_{i \in O} {}^2D_{i,w}^4 Y_{i,\delta}^{4,*} \tau_{\gamma,\delta,w}^2 \tau_{\gamma,\alpha,i}^5 \quad (4r_D r_T^2 r_V N_o) \quad (1826)$$

$$\tau_{\gamma,\delta,w}^7 = \sum_{i \in O} {}^2D_{i,w}^4 Y_{i,\gamma}^4 Y_{i,\delta}^{4,*} \quad (3r_D r_T^2 N_o) \quad (1814)$$

$$\tau_{\gamma,\delta,w}^8 = \sum_{\epsilon \in A} Z_{\delta,\epsilon}^* \tau_{\gamma,\epsilon,w}^6 \tau_{\gamma,\epsilon,w}^7 \quad (3r_D r_T^3) \quad (1815)$$

$$\tau_{\gamma,\alpha,w,i}^7 = \sum_{\delta \in A} \tau_{\delta,\alpha,i}^1 \tau_{\delta,\gamma,\alpha,w}^6 \quad (2r_D r_T^2 r_V N_o) \quad (1827)$$

$$\tau_{\gamma,w,i,j}^9 = \sum_{\delta \in A} \tau_{\delta,i,j}^5 \tau_{\delta,\gamma,w}^8 \quad (2r_D r_T^2 N_o^2) \quad (1816)$$

$$\tau_{\gamma,w,i,j}^8 = \sum_{\alpha \in B} W_{i,\alpha}^1 \tau_{\gamma,\alpha,w,j}^7 \quad (2r_D r_T r_V N_o^2) \quad (1828)$$

$$\tau_{\gamma,w,i}^9 = \sum_{\delta \in A} \sum_{j \in O} {}^2D_{j,w}^2 Y_{j,\gamma}^{2,*} Z_{\gamma,\delta}^* \tau_{\delta,w,i,j}^8 \quad (4r_D r_T^2 N_o^2) \quad \tau_{\gamma,w,i}^9 = \sum_{\delta \in A} \sum_{j \in O} {}^2D_{j,w}^2 Y_{j,\gamma}^{2,*} Z_{\gamma,\delta}^* \tau_{\delta,w,i,j}^8 \quad (4r_D r_T^2 N_o^2) \quad (1829) \quad (1841)$$

$${}^{21}R_{a,\gamma} \leftarrow \sum_{w \in D} \sum_{i \in O} \frac{1}{2} {}^2D_{a,w}^1 T_{a,i}^1 \tau_{\gamma,w,i}^9 \quad (3r_D r_T N_o N_v) \quad (1830)$$

Raw expression

$${}^{21}R_{a,\epsilon} \leftarrow \sum_{\gamma \in A} \sum_{i \in O} \sum_{j \in O} \sum_{k \in O} \sum_{l \in O} \sum_{b \in V} \sum_{c \in V} \sum_{d \in V} \frac{1}{2} \quad (1831)$$

$${}^1T_{c,i} \quad {}^1T_{d,k} \quad Y_{i,\epsilon}^{2,*} \quad Z_{\epsilon,\gamma}^* \quad Y_{b,\gamma}^{3,*} \quad Y_{j,\gamma}^{4,*} \quad {}^2D_{a,i,b,j} \quad {}^2T_{a,l,b,j} \quad V_{k,c,l,d}$$

Factorized expression

$$\tau_{\gamma,\alpha}^0 = \sum_{a \in V} W_{a,\alpha}^2 Y_{a,\gamma}^1 \quad (2r_T r_V N_v) \quad (1832)$$

$$\tau_{\gamma,\alpha,i}^1 = \sum_{\delta \in A} Y_{i,\delta}^2 Z_{\delta,\gamma} \tau_{\delta,\alpha}^0 \quad (3r_T^2 r_V N_o) \quad (1833)$$

$$\tau_{\gamma,\delta,w}^2 = \sum_{a \in V} {}^2D_{a,w}^3 Y_{a,\gamma}^3 Y_{a,\delta}^{3,*} \quad (3r_D r_T^2 N_v) \quad (1834)$$

$$\tau_{\alpha,i}^3 = \sum_{a \in V} {}^1T_{a,i} W_{a,\alpha}^4 \quad (2r_V N_o N_v) \quad (1835)$$

$$\tau_{\alpha,i,j}^4 = \sum_{\beta \in B} X_{\alpha,\beta} W_{j,\beta}^3 \tau_{\beta,i}^3 \quad (3r_V^2 N_o^2) \quad (1836)$$

$$\tau_{\gamma,\alpha,i}^5 = \sum_{j \in O} Y_{j,\gamma}^4 \tau_{\alpha,i,j}^4 \quad (2r_T r_V N_o^2) \quad (1837)$$

$$\tau_{\gamma,\delta,\alpha,w}^6 = \sum_{i \in O} {}^2D_{i,w}^4 Y_{i,\delta}^{4,*} \tau_{\gamma,\delta,w}^2 \tau_{\gamma,\alpha,i}^5 \quad (4r_D r_T^2 r_V N_o) \quad (1838)$$

$$\tau_{\gamma,\alpha,w,i}^7 = \sum_{\delta \in A} \tau_{\delta,\alpha,i}^1 \tau_{\delta,\gamma,\alpha,w}^6 \quad (2r_D r_T^2 r_V N_o) \quad (1839)$$

$$\tau_{\gamma,w,i,j}^8 = \sum_{\alpha \in B} W_{i,\alpha}^1 \tau_{\gamma,\alpha,w,j}^7 \quad (2r_D r_T r_V N_o^2) \quad (1840)$$

$${}^{21}R_{a,\gamma} \leftarrow \sum_{w \in D} \sum_{i \in O} \frac{1}{2} {}^2D_{a,w}^1 T_{a,i}^1 \tau_{\gamma,w,i}^9 \quad (3r_D r_T N_o N_v) \quad (1842)$$

Raw expression

$${}^{21}R_{a,\epsilon} \leftarrow \sum_{\gamma \in A} \sum_{i \in O} \sum_{j \in O} \sum_{k \in O} \sum_{l \in O} \sum_{b \in V} \sum_{c \in V} \sum_{d \in V} \frac{1}{2} \quad (1843)$$

$${}^1T_{c,i} \quad {}^1T_{d,k} \quad Y_{i,\epsilon}^{2,*} \quad Z_{\epsilon,\gamma}^* \quad Y_{b,\gamma}^{3,*} \quad Y_{j,\gamma}^{4,*} \quad {}^2D_{a,i,b,j} \quad {}^2T_{b,j,a,l} \quad V_{k,c,l,d}$$

Factorized expression

$$\tau_{\gamma,\delta,w}^0 = \sum_{a \in V} {}^2D_{a,w}^3 Y_{a,\gamma}^1 Y_{a,\delta}^{3,*} \quad (3r_D r_T^2 N_v) \quad (1844)$$

$$\tau_{\gamma,\delta,w}^1 = \sum_{i \in O} {}^2D_{i,w}^4 Y_{i,\gamma}^2 Y_{i,\delta}^{4,*} \quad (3r_D r_T^2 N_o) \quad (1845)$$

$$\tau_{\gamma,\delta,w}^2 = \sum_{\epsilon \in A} Z_{\delta,\epsilon}^* \tau_{\gamma,\epsilon,w}^0 \tau_{\gamma,\epsilon,w}^1 \quad (3r_D r_T^3) \quad (1846)$$

$$\tau_{\gamma,\delta,w}^3 = \sum_{\epsilon \in A} Z_{\epsilon,\gamma} \tau_{\epsilon,\delta,w}^2 \quad (2r_D r_T^3) \quad (1847)$$

$$\tau_{\gamma,\delta,w}^4 = \sum_{i \in O} {}^2D_{i,w}^2 Y_{i,\gamma}^4 Y_{i,\delta}^{2,*} \quad (3r_D r_T^2 N_o) \quad (1848)$$

$$\tau_{\alpha,i}^5 = \sum_{a \in V} {}^1T_{a,i} W_{a,\alpha}^2 \quad (2r_V N_o N_v) \quad (1849)$$

$$\tau_{\alpha,\beta}^6 = \sum_{i \in O} W_{i,\beta}^3 \tau_{\alpha,i}^5 \quad (2r_V^2 N_o) \quad (1850)$$

$$\tau_{\alpha,i}^7 = \sum_{\beta \in B} W_{i,\beta}^1 X_{\beta,\alpha} \tau_{\beta,\alpha}^6 \quad (3r_V^2 N_o) \quad (1851)$$

$$\tau_{i,a}^8 = \sum_{\alpha \in B} W_{a,\alpha}^4 \tau_{\alpha,i}^7 \quad (2r_V N_o N_v) \quad (1852)$$

$$\tau_{\gamma,i}^9 = \sum_{a \in V} Y_{a,\gamma}^3 \tau_{i,a}^8 \quad (2r_T N_o N_v) \quad (1853)$$

$$\tau^{10}_{\gamma,w,i} = \sum_{\delta \in A} \tau^9_{\delta,i} \tau^3_{\delta,\gamma,w} \tau^4_{\delta,\gamma,w} \quad (3r_D r_T^2 N_o) \quad (1854)$$

$$\tau^{10}_{\gamma,w,i} = \sum_{\delta \in A} \tau^9_{\delta,i} \tau^0_{\delta,\gamma,w} \tau^4_{\delta,\gamma,w} \quad (3r_D r_T^2 N_o) \quad (1867)$$

$${}^{21}R_{a,\gamma} \leftarrow \sum_{w \in D} \sum_{i \in O} \frac{1}{2} {}^2D^1_{a,w} {}^1T_{a,i} \tau^{10}_{\gamma,w,i} \quad (3r_D r_T N_o N_v) \quad (1855)$$

$${}^{21}R_{a,\gamma} \leftarrow \sum_{w \in D} \sum_{i \in O} \frac{1}{2} {}^2D^1_{a,w} {}^1T_{a,i} \tau^{10}_{\gamma,w,i} \quad (3r_D r_T N_o N_v) \quad (1868)$$

Raw expression

$${}^{21}R_{a,\epsilon} \leftarrow \sum_{\gamma \in A} \sum_{i \in O} \sum_{j \in O} \sum_{k \in O} \sum_{l \in O} \sum_{b \in V} \sum_{c \in V} \sum_{d \in V} \frac{1}{2} \quad (1856)$$

$$\begin{aligned} & {}^1T_{c,j} \quad {}^1T_{d,i} \quad Y^{2,*}_{i,\epsilon} \quad Z^*_{\epsilon,\gamma} \quad Y^{3,*}_{b,\gamma} \\ & Y^{4,*}_{j,\gamma} \quad {}^2D^{a,i,b,j} \quad {}^2T_{b,k,a,l} \quad V_{k,c,l,d} \end{aligned}$$

Raw expression

$${}^{21}R_{a,\epsilon} \leftarrow \sum_{\gamma \in A} \sum_{i \in O} \sum_{j \in O} \sum_{k \in O} \sum_{l \in O} \sum_{b \in V} \sum_{c \in V} \sum_{d \in V} \frac{1}{2} \quad (1869)$$

$$\begin{aligned} & {}^1T_{c,j} \quad {}^1T_{d,k} \quad Y^{2,*}_{i,\epsilon} \quad Z^*_{\epsilon,\gamma} \quad Y^{3,*}_{b,\gamma} \\ & Y^{4,*}_{j,\gamma} \quad {}^2D^{a,i,b,j} \quad {}^2T_{a,i,b,l} \quad V_{k,c,l,d} \end{aligned}$$

Factorized expression

$$\tau^0_{\gamma,\delta,w} = \sum_{i \in O} {}^2D^2_{i,w} Y^2_{i,\gamma} Y^{2,*}_{i,\delta} \quad (3r_D r_T^2 N_o) \quad (1857)$$

$$\tau^0_{\alpha,i} = \sum_{a \in V} {}^1T_{a,i} W^4_{a,\alpha} \quad (2r_V N_o N_v) \quad (1870)$$

$$\tau^1_{\gamma,\delta,w} = \sum_{a \in V} {}^2D^3_{a,w} Y^3_{a,\gamma} Y^{3,*}_{a,\delta} \quad (3r_D r_T^2 N_v) \quad (1858)$$

$$\tau^1_{\alpha,i,j} = \sum_{\beta \in B} X_{\alpha,\beta} W^3_{j,\beta} \tau^0_{\beta,i} \quad (3r_V^2 N_o^2) \quad (1871)$$

$$\tau^2_{\gamma,\delta,w} = \sum_{i \in O} {}^2D^4_{i,w} Y^4_{i,\gamma} Y^{4,*}_{i,\delta} \quad (3r_D r_T^2 N_o) \quad (1859)$$

$$\tau^2_{\gamma,\alpha,i} = \sum_{j \in O} Y^2_{j,\gamma} \tau^1_{\alpha,i,j} \quad (2r_T r_V N_o^2) \quad (1872)$$

$$\tau^3_{\gamma,\delta,w} = \sum_{\epsilon \in A} Z^*_{\delta,\epsilon} \tau^1_{\gamma,\epsilon,w} \tau^2_{\gamma,\epsilon,w} \quad (3r_D r_T^3) \quad (1860)$$

$$\tau^3_{\gamma,w,i} = \sum_{a \in V} {}^2D^3_{a,w} {}^1T_{a,i} Y^{3,*}_{a,\gamma} \quad (3r_D r_T N_o N_v) \quad (1873)$$

$$\tau^4_{\gamma,\delta,w} = \sum_{\epsilon \in A} Z_{\gamma,\epsilon} \tau^3_{\epsilon,\delta,w} \quad (2r_D r_T^3) \quad (1861)$$

$$\tau^4_{\gamma,w,i,j} = \sum_{\delta \in A} {}^2D^4_{i,w} Z^*_{\gamma,\delta} Y^{4,*}_{i,\delta} \tau^3_{\delta,w,j} \quad (4r_D r_T^2 N_o^2) \quad (1874)$$

$$\tau^5_{\alpha,i} = \sum_{a \in V} {}^1T_{a,i} W^2_{a,\alpha} \quad (2r_V N_o N_v) \quad (1862)$$

$$\tau^5_{\gamma,\alpha,w,i} = \sum_{j \in O} W^1_{j,\alpha} \tau^4_{\gamma,w,i,j} \quad (2r_D r_T r_V N_o^2) \quad (1875)$$

$$\tau^6_{\alpha,\beta} = \sum_{i \in O} W^3_{i,\beta} \tau^5_{\alpha,i} \quad (2r_V^2 N_o) \quad (1863)$$

$$\tau^6_{\gamma,\alpha} = \sum_{a \in V} W^2_{a,\alpha} Y^3_{a,\gamma} \quad (2r_T r_V N_v) \quad (1876)$$

$$\tau^7_{\alpha,i} = \sum_{\beta \in B} W^1_{i,\beta} X_{\beta,\alpha} \tau^6_{\beta,\alpha} \quad (3r_V^2 N_o) \quad (1864)$$

$$\tau^7_{\gamma,\alpha,i} = \sum_{\delta \in A} Z_{\gamma,\delta} Y^4_{i,\delta} \tau^6_{\delta,\alpha} \quad (3r_T^2 r_V N_o) \quad (1877)$$

$$\tau^8_{i,a} = \sum_{\alpha \in B} W^4_{a,\alpha} \tau^7_{\alpha,i} \quad (2r_V N_o N_v) \quad (1865)$$

$$\tau^9_{\gamma,i} = \sum_{a \in V} Y^1_{a,\gamma} \tau^8_{i,a} \quad (2r_T N_o N_v) \quad (1866)$$

$$\tau^8_{\gamma,\delta,\alpha,w} = \sum_{i \in O} \tau^7_{\gamma,\alpha,i} \tau^5_{\delta,\alpha,w,i} \quad (2r_D r_T^2 r_V N_o) \quad (1878)$$

$$\tau_{\gamma,\delta,w,i}^9 = \sum_{\alpha \in B} \tau_{\gamma,\alpha,i}^2 \tau_{\gamma,\delta,\alpha,w}^8 \quad (2r_D r_T^2 r_V N_o) \quad (1879)$$

$$\tau_{\gamma,\delta,\alpha,w}^8 = \sum_{i \in O} \tau_{\gamma,\alpha,i}^7 \tau_{\delta,\alpha,w,i}^5 \quad (2r_D r_T^2 r_V N_o) \quad (1891)$$

$$\tau_{\gamma,\delta,w}^{10} = \sum_{i \in O} {}^2D_{i,w}^2 Y_{i,\delta}^{2,*} \tau_{\gamma,\delta,w,i}^9 \quad (3r_D r_T^2 N_o) \quad (1880)$$

$$\tau_{\gamma,\delta,w,i}^9 = \sum_{\alpha \in B} \tau_{\gamma,\alpha,i}^2 \tau_{\gamma,\delta,\alpha,w}^8 \quad (2r_D r_T^2 r_V N_o) \quad (1892)$$

$${}^{21}R_{a,\gamma} \leftarrow \sum_{\delta \in A} \sum_{w \in D} \frac{1}{2} {}^2D_{a,w}^1 Y_{a,\delta}^1 \tau_{\delta,\gamma,w}^{10} \quad (3r_D r_T^2 N_v) \quad (1881)$$

$$\tau_{\gamma,\delta,w}^{10} = \sum_{i \in O} {}^2D_{i,w}^2 Y_{i,\delta}^{2,*} \tau_{\gamma,\delta,w,i}^9 \quad (3r_D r_T^2 N_o) \quad (1893)$$

Raw expression

$${}^{21}R_{a,\epsilon} \leftarrow \sum_{\gamma \in A} \sum_{i \in O} \sum_{j \in O} \sum_{k \in O} \sum_{l \in O} \sum_{b \in V} \sum_{c \in V} \sum_{d \in V} \frac{1}{2} \quad (1882)$$

$$\begin{aligned} & {}^1T_{c,j} \quad {}^1T_{d,k} \quad Y_{i,\epsilon}^{2,*} \quad Z_{\epsilon,\gamma}^* \quad Y_{b,\gamma}^{3,*} \\ & Y_{j,\gamma}^{4,*} \quad {}^2D_{a,i,b,j} \quad {}^2T_{b,l,a,i} \quad V_{k,c,l,d} \end{aligned}$$

$${}^{21}R_{a,\gamma} \leftarrow \sum_{\delta \in A} \sum_{w \in D} \frac{1}{2} {}^2D_{a,w}^1 Y_{a,\delta}^3 \tau_{\delta,\gamma,w}^{10} \quad (3r_D r_T^2 N_v) \quad (1894)$$

Raw expression

$${}^{21}R_{a,\epsilon} \leftarrow - \sum_{\gamma \in A} \sum_{i \in O} \sum_{j \in O} \sum_{k \in O} \sum_{l \in O} \sum_{b \in V} \sum_{c \in V} \sum_{d \in V} {}^1T_{a,k}$$

$$\begin{aligned} & {}^1T_{c,i} \quad Y_{i,\epsilon}^{2,*} \quad Z_{\epsilon,\gamma}^* \quad Y_{b,\gamma}^{3,*} \\ & Y_{j,\gamma}^{4,*} \quad {}^2D_{a,i,b,j} \quad {}^2T_{b,j,d,l} \quad V_{k,c,l,d} \end{aligned} \quad (1895)$$

Factorized expression

$$\tau_{\alpha,i}^0 = \sum_{a \in V} {}^1T_{a,i} W_{a,\alpha}^4 \quad (2r_V N_o N_v) \quad (1883)$$

Factorized expression

$$\tau_{\alpha,i,j}^1 = \sum_{\beta \in B} X_{\alpha,\beta} W_{j,\beta}^3 \tau_{\beta,i}^0 \quad (3r_V^2 N_o^2) \quad (1884)$$

$$\tau_{\gamma,\alpha}^0 = \sum_{i \in O} W_{i,\alpha}^3 Y_{i,\gamma}^2 \quad (2r_T r_V N_o) \quad (1896)$$

$$\tau_{\gamma,\alpha,i}^2 = \sum_{j \in O} Y_{j,\gamma}^4 \tau_{\alpha,i,j}^1 \quad (2r_T r_V N_o^2) \quad (1885)$$

$$\tau_{\gamma,\alpha}^1 = \sum_{a \in V} W_{a,\alpha}^4 Y_{a,\gamma}^3 \quad (2r_T r_V N_v) \quad (1897)$$

$$\tau_{\gamma,w,i}^3 = \sum_{a \in V} {}^2D_{a,w}^3 {}^1T_{a,i} Y_{a,\gamma}^{3,*} \quad (3r_D r_T N_o N_v) \quad (1886)$$

$$\tau_{\gamma,\alpha,i}^2 = \sum_{\delta \in A} Z_{\gamma,\delta} Y_{i,\delta}^4 \tau_{\delta,\alpha}^1 \quad (3r_T^2 r_V N_o) \quad (1898)$$

$$\tau_{\gamma,w,i,j}^4 = \sum_{\delta \in A} {}^2D_{i,w}^4 Z_{\gamma,\delta}^* Y_{i,\delta}^{4,*} \tau_{\delta,w,j}^3 \quad (4r_D r_T^2 N_o^2) \quad (1887)$$

$$\tau_{\alpha,i}^3 = \sum_{a \in V} {}^1T_{a,i} W_{a,\alpha}^2 \quad (2r_V N_o N_v) \quad (1899)$$

$$\tau_{\gamma,\alpha,w,i}^5 = \sum_{j \in O} W_{j,\alpha}^1 \tau_{\gamma,w,i,j}^4 \quad (2r_D r_T r_V N_o^2) \quad (1888)$$

$$\tau_{\gamma,\alpha,w}^4 = \sum_{i \in O} {}^2D_{i,w}^4 Y_{i,\gamma}^{4,*} \tau_{\alpha,i}^3 \quad (3r_D r_T r_V N_o) \quad (1900)$$

$$\tau_{\gamma,\alpha}^6 = \sum_{a \in V} W_{a,\alpha}^2 Y_{a,\gamma}^1 \quad (2r_T r_V N_v) \quad (1889)$$

$$\tau_{\gamma,w,i}^5 = \sum_{a \in V} {}^2D_{a,w}^3 {}^1T_{a,i} Y_{a,\gamma}^{3,*} \quad (3r_D r_T N_o N_v) \quad (1901)$$

$$\tau_{\gamma,\alpha,i}^7 = \sum_{\delta \in A} Y_{i,\delta}^2 Z_{\delta,\gamma} \tau_{\delta,\alpha}^6 \quad (3r_T^2 r_V N_o) \quad (1890)$$

$$\tau_{\gamma,\alpha,w}^6 = \sum_{i \in O} W_{i,\alpha}^1 \tau_{\gamma,w,i}^5 \quad (2r_D r_T r_V N_o) \quad (1902)$$

$$\tau^7_{\gamma,\alpha,w} = \sum_{\beta \in B} X_{\beta,\alpha} \tau^4_{\gamma,\beta,w} \tau^6_{\gamma,\beta,w} \quad (3r_D r_T r_V^2) \quad (1903)$$

$$\tau^8_{\gamma,\alpha,w} = \sum_{\delta \in A} Z^*_{\gamma,\delta} \tau^7_{\delta,\alpha,w} \quad (2r_D r_T^2 r_V) \quad (1904)$$

$$\tau^9_{\gamma,\delta,w,i} = \sum_{\alpha \in B} \tau^0_{\gamma,\alpha} \tau^2_{\gamma,\alpha,i} \tau^8_{\delta,\alpha,w} \quad (3r_D r_T^2 r_V N_o) \quad (1905)$$

$$\tau^{10}_{\gamma,\delta,w} = \sum_{i \in O} {}^2D^2_{i,w} Y^{2,*}_{i,\delta} \tau^9_{\gamma,\delta,w,i} \quad (3r_D r_T^2 N_o) \quad (1906)$$

$${}^{21}R_{a,\gamma} \leftarrow \sum_{\delta \in A} \sum_{w \in D} \frac{1}{2} {}^2D^1_{a,w} Y^1_{a,\delta} \tau^{10}_{\delta,\gamma,w} \quad (3r_D r_T^2 N_v) \quad (1907)$$

Raw expression

$${}^{21}R_{a,\epsilon} \leftarrow - \sum_{\gamma \in A} \sum_{i \in O} \sum_{j \in O} \sum_{k \in O} \sum_{l \in O} \sum_{b \in V} \sum_{c \in V} \sum_{d \in V} {}^1T_{a,k} \\ {}^1T_{c,i} Y^{2,*}_{i,\epsilon} Z^*_{\epsilon,\gamma} Y^{3,*}_{b,\gamma} Y^{4,*}_{j,\gamma} {}^2D^{a,i,b,j} {}^2T_{d,l,b,j} V_{k,c,l,d} \quad (1908)$$

Factorized expression

$$\tau^0_{\gamma,\alpha} = \sum_{a \in V} W^4_{a,\alpha} Y^1_{a,\gamma} \quad (2r_T r_V N_v) \quad (1909)$$

$$\tau^1_{\gamma,\alpha,i} = \sum_{\delta \in A} Y^2_{i,\delta} Z_{\delta,\gamma} \tau^0_{\delta,\alpha} \quad (3r_T^2 r_V N_o) \quad (1910)$$

$$\tau^2_{\gamma,\alpha} = \sum_{i \in O} W^3_{i,\alpha} Y^4_{i,\gamma} \quad (2r_T r_V N_o) \quad (1911)$$

$$\tau^3_{\alpha,i} = \sum_{a \in V} {}^1T_{a,i} W^2_{a,\alpha} \quad (2r_V N_o N_v) \quad (1912)$$

$$\tau^4_{\gamma,\alpha,w} = \sum_{i \in O} {}^2D^4_{i,w} Y^{4,*}_{i,\gamma} \tau^3_{\alpha,i} \quad (3r_D r_T r_V N_o) \quad (1913)$$

$$\tau^5_{\gamma,w,i} = \sum_{a \in V} {}^2D^3_{a,w} {}^1T_{a,i} Y^{3,*}_{a,\gamma} \quad (3r_D r_T N_o N_v) \quad (1914)$$

$$\tau^6_{\gamma,\alpha,w} = \sum_{i \in O} W^1_{i,\alpha} \tau^5_{\gamma,w,i} \quad (2r_D r_T r_V N_o) \quad (1915)$$

$$\tau^7_{\gamma,\alpha,w} = \sum_{\beta \in B} X_{\beta,\alpha} \tau^4_{\gamma,\beta,w} \tau^6_{\gamma,\beta,w} \quad (3r_D r_T r_V^2) \quad (1916)$$

$$\tau^8_{\gamma,\alpha,w} = \sum_{\delta \in A} Z^*_{\gamma,\delta} \tau^7_{\delta,\alpha,w} \quad (2r_D r_T^2 r_V) \quad (1917)$$

$$\tau^9_{\gamma,\delta,w,i} = \sum_{\alpha \in B} \tau^2_{\gamma,\alpha} \tau^1_{\gamma,\alpha,i} \tau^8_{\delta,\alpha,w} \quad (3r_D r_T^2 r_V N_o) \quad (1918)$$

$$\tau^{10}_{\gamma,\delta,w} = \sum_{i \in O} {}^2D^2_{i,w} Y^{2,*}_{i,\delta} \tau^9_{\gamma,\delta,w,i} \quad (3r_D r_T^2 N_o) \quad (1919)$$

$${}^{21}R_{a,\gamma} \leftarrow \sum_{\delta \in A} \sum_{w \in D} \frac{1}{2} {}^2D^1_{a,w} Y^3_{a,\delta} \tau^{10}_{\delta,\gamma,w} \quad (3r_D r_T^2 N_v) \quad (1920)$$

Raw expression

$${}^{21}R_{a,\epsilon} \leftarrow - \sum_{\gamma \in A} \sum_{i \in O} \sum_{j \in O} \sum_{k \in O} \sum_{l \in O} \sum_{b \in V} \sum_{c \in V} \sum_{d \in V} {}^1T_{a,k} \\ {}^1T_{c,l} Y^{2,*}_{i,\epsilon} Z^*_{\epsilon,\gamma} Y^{3,*}_{b,\gamma} Y^{4,*}_{j,\gamma} {}^2D^{a,i,b,j} {}^2T_{b,j,d,i} V_{k,d,l,c} \quad (1921)$$

Factorized expression

$$\tau^0_{\gamma,\delta,w} = \sum_{i \in O} {}^2D^2_{i,w} Y^2_{i,\gamma} Y^{2,*}_{i,\delta} \quad (3r_D r_T^2 N_o) \quad (1922)$$

$$\tau^1_{\gamma,w,i} = \sum_{a \in V} {}^2D^3_{a,w} {}^1T_{a,i} Y^{3,*}_{a,\gamma} \quad (3r_D r_T N_o N_v) \quad (1923)$$

$$\tau^2_{\gamma,\alpha} = \sum_{a \in V} W^2_{a,\alpha} Y^3_{a,\gamma} \quad (2r_T r_V N_v) \quad (1924)$$

$$\tau^3_{\alpha,i} = \sum_{a \in V} {}^1T_{a,i} W^4_{a,\alpha} \quad (2r_V N_o N_v) \quad (1925)$$

$$\tau^4_{\alpha,i,j} = \sum_{\beta \in B} X_{\alpha,\beta} W^3_{j,\beta} \tau^3_{\beta,i} \quad (3r_V^2 N_o^2) \quad (1926)$$

$$\tau^5_{\gamma,\alpha,i} = \sum_{j \in O} Y^4_{j,\gamma} \tau^4_{\alpha,i,j} \quad (2r_T r_V N_o^2) \quad (1927)$$

$$\tau^5_{\gamma,\alpha,i} = \sum_{j \in O} Y^2_{j,\gamma} \tau^4_{\alpha,i,j} \quad (2r_T r_V N_o^2) \quad (1939)$$

$$\tau^6_{\gamma,i,j} = \sum_{\alpha \in B} W^1_{j,\alpha} \tau^2_{\gamma,\alpha} \tau^5_{\gamma,\alpha,i} \quad (3r_T r_V N_o^2) \quad (1928)$$

$$\tau^6_{\gamma,i,j} = \sum_{\alpha \in B} W^1_{j,\alpha} \tau^2_{\gamma,\alpha} \tau^5_{\gamma,\alpha,i} \quad (3r_T r_V N_o^2) \quad (1940)$$

$$\tau^7_{\gamma,i,j} = \sum_{\delta \in A} Z_{\gamma,\delta} \tau^6_{\delta,i,j} \quad (2r_T^2 N_o^2) \quad (1929)$$

$$\tau^7_{\gamma,i,j} = \sum_{\delta \in A} Z_{\delta,\gamma} \tau^6_{\delta,i,j} \quad (2r_T^2 N_o^2) \quad (1941)$$

$$\tau^8_{\gamma,\delta,w} = \sum_{i \in O} \sum_{j \in O} {}^2D^4_{i,w} Y^{4,*}_{i,\delta} \tau^1_{\delta,w,j} \tau^7_{\gamma,i,j} \quad (4r_D r_T^2 N_o^2) \quad (1930)$$

$$\tau^8_{\gamma,\delta,w} = \sum_{i \in O} \sum_{j \in O} {}^2D^4_{i,w} Y^{4,*}_{i,\delta} \tau^1_{\delta,w,j} \tau^7_{\gamma,i,j} \quad (4r_D r_T^2 N_o^2) \quad (1942)$$

$$\tau^9_{\gamma,\delta,w} = \sum_{\epsilon \in A} Z^*_{\delta,\epsilon} \tau^8_{\gamma,\epsilon,w} \quad (2r_D r_T^3) \quad (1931)$$

$$\tau^9_{\gamma,\delta,w} = \sum_{\epsilon \in A} Z^*_{\delta,\epsilon} \tau^8_{\gamma,\epsilon,w} \quad (2r_D r_T^3) \quad (1943)$$

$${}^{21}R_{a,\gamma} \leftarrow \sum_{\delta \in A} \sum_{w \in D} \frac{1}{2} {}^2D^1_{a,w} Y^1_{a,\delta} \tau^0_{\delta,\gamma,w} \tau^9_{\delta,\gamma,w} \quad (4r_D r_T^2 N_v) \quad (1932)$$

$${}^{21}R_{a,\gamma} \leftarrow \sum_{\delta \in A} \sum_{w \in D} \frac{1}{2} {}^2D^1_{a,w} Y^3_{a,\delta} \tau^0_{\delta,\gamma,w} \tau^9_{\delta,\gamma,w} \quad (4r_D r_T^2 N_v) \quad (1944)$$

Raw expression

$${}^{21}R_{a,\epsilon} \leftarrow - \sum_{\gamma \in A} \sum_{i \in O} \sum_{j \in O} \sum_{k \in O} \sum_{l \in O} \sum_{b \in V} \sum_{c \in V} \sum_{d \in V} {}^1T_{a,k} \\ {}^1T_{c,l} Y^{2,*}_{i,\epsilon} Z^*_{\epsilon,\gamma} Y^{3,*}_{b,\gamma} \\ Y^{4,*}_{j,\gamma} {}^2D^{a,i,b,j} {}^2T_{d,i,b,j} V_{k,d,l,c} \quad (1933)$$

Raw expression

$${}^{21}R_{a,\epsilon} \leftarrow - \sum_{\gamma \in A} \sum_{i \in O} \sum_{j \in O} \sum_{k \in O} \sum_{l \in O} \sum_{b \in V} \sum_{c \in V} \sum_{d \in V} {}^1T_{b,k} \\ {}^1T_{c,j} Y^{2,*}_{i,\epsilon} Z^*_{\epsilon,\gamma} Y^{3,*}_{b,\gamma} \\ Y^{4,*}_{j,\gamma} {}^2D^{a,i,b,j} {}^2T_{a,i,d,l} V_{k,c,l,d} \quad (1945)$$

Factorized expression

$$\tau^0_{\gamma,\delta,w} = \sum_{i \in O} {}^2D^2_{i,w} Y^4_{i,\gamma} Y^{2,*}_{i,\delta} \quad (3r_D r_T^2 N_o) \quad (1934)$$

Factorized expression

$$\tau^0_{\gamma,\delta,w} = \sum_{i \in O} {}^2D^2_{i,w} Y^2_{i,\gamma} Y^{2,*}_{i,\delta} \quad (3r_D r_T^2 N_o) \quad (1946)$$

$$\tau^1_{\gamma,w,i} = \sum_{a \in V} {}^2D^3_{a,w} {}^1T_{a,i} Y^{3,*}_{a,\gamma} \quad (3r_D r_T N_o N_v) \quad (1935)$$

$$\tau^1_{\gamma,\delta,w} = \sum_{i \in O} {}^2D^4_{i,w} Y^4_{i,\gamma} Y^{4,*}_{i,\delta} \quad (3r_D r_T^2 N_o) \quad (1947)$$

$$\tau^2_{\gamma,\alpha} = \sum_{a \in V} W^2_{a,\alpha} Y^1_{a,\gamma} \quad (2r_T r_V N_v) \quad (1936)$$

$$\tau^2_{\gamma,w,i} = \sum_{a \in V} {}^2D^3_{a,w} {}^1T_{a,i} Y^{3,*}_{a,\gamma} \quad (3r_D r_T N_o N_v) \quad (1948)$$

$$\tau^3_{\alpha,i} = \sum_{a \in V} {}^1T_{a,i} W^4_{a,\alpha} \quad (2r_V N_o N_v) \quad (1937)$$

$$\tau^3_{\alpha,i} = \sum_{a \in V} {}^1T_{a,i} W^2_{a,\alpha} \quad (2r_V N_o N_v) \quad (1949)$$

$$\tau^4_{\alpha,i,j} = \sum_{\beta \in B} X_{\alpha,\beta} W^3_{j,\beta} \tau^3_{\beta,i} \quad (3r_V^2 N_o^2) \quad (1938)$$

$$\tau^4_{\alpha,\beta} = \sum_{i \in O} W^3_{i,\beta} \tau^3_{\alpha,i} \quad (2r_V^2 N_o) \quad (1950)$$

$$\tau^5_{\alpha,i} = \sum_{\beta \in B} W^1_{i,\beta} X_{\beta,\alpha} \tau^4_{\beta,\alpha} \quad (3r_V^2 N_o) \quad (1951)$$

$$\tau^5_{\alpha,i} = \sum_{\beta \in B} W^1_{i,\beta} X_{\beta,\alpha} \tau^4_{\beta,\alpha} \quad (3r_V^2 N_o) \quad (1964)$$

$$\tau^6_{i,a} = \sum_{\alpha \in B} W^4_{a,\alpha} \tau^5_{\alpha,i} \quad (2r_V N_o N_v) \quad (1952)$$

$$\tau^6_{i,a} = \sum_{\alpha \in B} W^4_{a,\alpha} \tau^5_{\alpha,i} \quad (2r_V N_o N_v) \quad (1965)$$

$$\tau^7_{\gamma,i} = \sum_{a \in V} Y^3_{a,\gamma} \tau^6_{i,a} \quad (2r_T N_o N_v) \quad (1953)$$

$$\tau^7_{\gamma,i} = \sum_{a \in V} Y^1_{a,\gamma} \tau^6_{i,a} \quad (2r_T N_o N_v) \quad (1966)$$

$$\tau^8_{\gamma,\delta,w} = \sum_{i \in O} \tau^7_{\gamma,i} \tau^2_{\delta,w,i} \quad (2r_D r_T^2 N_o) \quad (1954)$$

$$\tau^8_{\gamma,\delta,w} = \sum_{i \in O} \tau^7_{\gamma,i} \tau^2_{\delta,w,i} \quad (2r_D r_T^2 N_o) \quad (1967)$$

$$\tau^9_{\gamma,\delta,w} = \sum_{\epsilon \in A} Z^*_{\delta,\epsilon} \tau^1_{\gamma,\epsilon,w} \tau^8_{\gamma,\epsilon,w} \quad (3r_D r_T^3) \quad (1955)$$

$$\tau^9_{\gamma,\delta,w} = \sum_{\epsilon \in A} Z^*_{\delta,\epsilon} \tau^1_{\gamma,\epsilon,w} \tau^8_{\gamma,\epsilon,w} \quad (3r_D r_T^3) \quad (1968)$$

$$\tau^{10}_{\gamma,\delta,w} = \sum_{\epsilon \in A} Z_{\gamma,\epsilon} \tau^9_{\epsilon,\delta,w} \quad (2r_D r_T^3) \quad (1956)$$

$$\tau^{10}_{\gamma,\delta,w} = \sum_{\epsilon \in A} Z_{\epsilon,\gamma} \tau^9_{\epsilon,\delta,w} \quad (2r_D r_T^3) \quad (1969)$$

$${}^{21}R_{a,\gamma} \leftarrow \sum_{\delta \in A} \sum_{w \in D} \frac{1}{2} {}^2D^1_{a,w} Y^1_{a,\delta} \tau^0_{\delta,\gamma,w} \tau^{10}_{\delta,\gamma,w} \quad (4r_D r_T^2 N_v) \quad (1957)$$

$${}^{21}R_{a,\gamma} \leftarrow \sum_{\delta \in A} \sum_{w \in D} \frac{1}{2} {}^2D^1_{a,w} Y^3_{a,\delta} \tau^0_{\delta,\gamma,w} \tau^{10}_{\delta,\gamma,w} \quad (4r_D r_T^2 N_v) \quad (1970)$$

Raw expression

$${}^{21}R_{a,\epsilon} \leftarrow - \sum_{\gamma \in A} \sum_{i \in O} \sum_{j \in O} \sum_{k \in O} \sum_{l \in O} \sum_{b \in V} \sum_{c \in V} \sum_{d \in V} {}^1T_{b,k} \\ {}^1T_{c,j} Y^{2,*}_{i,\epsilon} Z^*_{\epsilon,\gamma} Y^{3,*}_{b,\gamma} \\ Y^{4,*}_{j,\gamma} {}^2D^{a,i,b,j} {}^2T_{d,l,a,i} V_{k,c,l,d} \quad (1958)$$

Raw expression

$${}^{21}R_{a,\epsilon} \leftarrow - \sum_{\gamma \in A} \sum_{i \in O} \sum_{j \in O} \sum_{k \in O} \sum_{l \in O} \sum_{b \in V} \sum_{c \in V} \sum_{d \in V} {}^1T_{b,k} \\ {}^1T_{c,l} Y^{2,*}_{i,\epsilon} Z^*_{\epsilon,\gamma} Y^{3,*}_{b,\gamma} \\ Y^{4,*}_{j,\gamma} {}^2D^{a,i,b,j} {}^2T_{a,i,d,j} V_{k,d,l,c} \quad (1971)$$

Factorized expression

$$\tau^0_{\gamma,\delta,w} = \sum_{i \in O} {}^2D^2_{i,w} Y^4_{i,\gamma} Y^{2,*}_{i,\delta} \quad (3r_D r_T^2 N_o) \quad (1959)$$

$$\tau^0_{\alpha,i} = \sum_{a \in V} {}^1T_{a,i} W^4_{a,\alpha} \quad (2r_V N_o N_v) \quad (1972)$$

$$\tau^1_{\gamma,\delta,w} = \sum_{i \in O} {}^2D^4_{i,w} Y^2_{i,\gamma} Y^{4,*}_{i,\delta} \quad (3r_D r_T^2 N_o) \quad (1960)$$

$$\tau^1_{\gamma,\alpha,w} = \sum_{i \in O} {}^2D^4_{i,w} Y^{4,*}_{i,\gamma} \tau^0_{\alpha,i} \quad (3r_D r_T r_V N_o) \quad (1973)$$

$$\tau^2_{\gamma,w,i} = \sum_{a \in V} {}^2D^3_{a,w} {}^1T_{a,i} Y^{3,*}_{a,\gamma} \quad (3r_D r_T N_o N_v) \quad (1961)$$

$$\tau^2_{\gamma,\delta,w} = \sum_{a \in V} {}^2D^3_{a,w} Y^3_{a,\gamma} Y^{3,*}_{a,\delta} \quad (3r_D r_T^2 N_v) \quad (1974)$$

$$\tau^3_{\alpha,i} = \sum_{a \in V} {}^1T_{a,i} W^2_{a,\alpha} \quad (2r_V N_o N_v) \quad (1962)$$

$$\tau^3_{\gamma,\delta,w,i} = \sum_{\epsilon \in A} Z_{\gamma,\epsilon} Y^4_{i,\epsilon} \tau^2_{\epsilon,\delta,w} \quad (3r_D r_T^3 N_o) \quad (1975)$$

$$\tau^4_{\alpha,\beta} = \sum_{i \in O} W^3_{i,\beta} \tau^3_{\alpha,i} \quad (2r_V^2 N_o) \quad (1963)$$

$$\tau^4_{\gamma,\delta,\alpha,w} = \sum_{i \in O} W^3_{i,\alpha} \tau^1_{\delta,\alpha,w} \tau^3_{\gamma,\delta,w,i} \quad (3r_D r_T^2 r_V N_o) \quad (1976)$$

$$\tau^5_{\alpha,i} = \sum_{a \in V} {}^1T_{a,i} W^2_{a,\alpha} \quad (2r_V N_o N_v) \quad (1977)$$

$$\tau^6_{\alpha,i,j} = \sum_{\beta \in B} W^1_{j,\beta} X_{\beta,\alpha} \tau^5_{\beta,i} \quad (3r_V^2 N_o^2) \quad (1978)$$

$$\tau^7_{\gamma,\alpha,i} = \sum_{j \in O} Y^2_{j,\gamma} \tau^6_{\alpha,i,j} \quad (2r_T r_V N_o^2) \quad (1979)$$

$$\tau^8_{\gamma,\delta,w,i} = \sum_{\alpha \in B} \tau^7_{\gamma,\alpha,i} \tau^4_{\gamma,\delta,\alpha,w} \quad (2r_D r_T^2 r_V N_o) \quad (1980)$$

$$\tau^9_{\gamma,\delta,w} = \sum_{\epsilon \in A} \sum_{i \in O} {}^2D^2_{i,w} Y^{2,*}_{i,\delta} Z^*_{\delta,\epsilon} \tau^8_{\gamma,\epsilon,w,i} \quad (4r_D r_T^3 N_o) \quad (1981)$$

$${}^{21}R_{a,\gamma} \leftarrow \sum_{\delta \in A} \sum_{w \in D} \frac{1}{2} {}^2D^1_{a,w} Y^1_{a,\delta} \tau^9_{\delta,\gamma,w} \quad (3r_D r_T^2 N_v) \quad (1982)$$

Raw expression

$${}^{21}R_{a,\epsilon} \leftarrow - \sum_{\gamma \in A} \sum_{i \in O} \sum_{j \in O} \sum_{k \in O} \sum_{l \in O} \sum_{b \in V} \sum_{c \in V} \sum_{d \in V} {}^1T_{b,k} \\ {}^1T_{c,l} Y^{2,*}_{i,\epsilon} Z^*_{\epsilon,\gamma} Y^{3,*}_{b,\gamma} \\ Y^{4,*}_{j,\gamma} {}^2D^{a,i,b,j} {}^2T_{d,j,a,i} V_{k,d,l,c} \quad (1983)$$

Factorized expression

$$\tau^0_{\gamma,\delta,w} = \sum_{a \in V} {}^2D^3_{a,w} Y^3_{a,\gamma} Y^{3,*}_{a,\delta} \quad (3r_D r_T^2 N_v) \quad (1984)$$

$$\tau^1_{\gamma,\delta,w} = \sum_{i \in O} {}^2D^4_{i,w} Y^4_{i,\gamma} Y^{4,*}_{i,\delta} \quad (3r_D r_T^2 N_o) \quad (1985)$$

$$\tau^2_{\gamma,\delta,w} = \sum_{\epsilon \in A} Z^*_{\delta,\epsilon} \tau^0_{\gamma,\epsilon,w} \tau^1_{\gamma,\epsilon,w} \quad (3r_D r_T^3) \quad (1986)$$

$$\tau^3_{\gamma,\delta,w} = \sum_{\epsilon \in A} Z_{\gamma,\epsilon} \tau^2_{\epsilon,\delta,w} \quad (2r_D r_T^3) \quad (1987)$$

$$\tau^4_{\alpha,i} = \sum_{a \in V} {}^1T_{a,i} W^4_{a,\alpha} \quad (2r_V N_o N_v) \quad (1988)$$

$$\tau^5_{\alpha,\beta} = \sum_{i \in O} W^1_{i,\alpha} \tau^4_{\beta,i} \quad (2r_V^2 N_o) \quad (1989)$$

$$\tau^6_{\alpha,i} = \sum_{\beta \in B} X_{\alpha,\beta} W^3_{i,\beta} \tau^5_{\alpha,\beta} \quad (3r_V^2 N_o) \quad (1990)$$

$$\tau^7_{i,a} = \sum_{\alpha \in B} W^2_{a,\alpha} \tau^6_{\alpha,i} \quad (2r_V N_o N_v) \quad (1991)$$

$$\tau^8_{i,j} = \sum_{a \in V} {}^1T_{a,i} \tau^7_{j,a} \quad (2N_o^2 N_v) \quad (1992)$$

$$\tau^9_{\gamma,i} = \sum_{j \in O} Y^2_{j,\gamma} \tau^8_{i,j} \quad (2r_T N_o^2) \quad (1993)$$

$$\tau^{10}_{\gamma,\delta,w} = \sum_{i \in O} {}^2D^2_{i,w} Y^{2,*}_{i,\delta} \tau^9_{\gamma,i} \quad (3r_D r_T^2 N_o) \quad (1994)$$

$${}^{21}R_{a,\gamma} \leftarrow \sum_{\delta \in A} \sum_{w \in D} \frac{1}{2} {}^2D^1_{a,w} Y^1_{a,\delta} \tau^{10}_{\delta,\gamma,w} \tau^3_{\delta,\gamma,w} \quad (4r_D r_T^2 N_v) \quad (1995)$$

Raw expression

$${}^{21}R_{a,\epsilon} \leftarrow - \sum_{\gamma \in A} \sum_{i \in O} \sum_{j \in O} \sum_{k \in O} \sum_{l \in O} \sum_{b \in V} \sum_{c \in V} \sum_{d \in V} {}^1T_{c,k} \\ {}^1T_{d,i} Y^{2,*}_{i,\epsilon} Z^*_{\epsilon,\gamma} Y^{3,*}_{b,\gamma} \\ Y^{4,*}_{j,\gamma} {}^2D^{a,i,b,j} {}^2T_{a,l,b,j} V_{k,c,l,d} \quad (1996)$$

Factorized expression

$$\tau^0_{\gamma,\delta,w} = \sum_{a \in V} {}^2D^3_{a,w} Y^1_{a,\gamma} Y^{3,*}_{a,\delta} \quad (3r_D r_T^2 N_v) \quad (1997)$$

$$\tau^1_{\gamma,\delta,w} = \sum_{i \in O} {}^2D^4_{i,w} Y^2_{i,\gamma} Y^{4,*}_{i,\delta} \quad (3r_D r_T^2 N_o) \quad (1998)$$

$$\tau^2_{\gamma,\delta,w} = \sum_{\epsilon \in A} Z^*_{\delta,\epsilon} \tau^0_{\gamma,\epsilon,w} \tau^1_{\gamma,\epsilon,w} \quad (3r_D r_T^3) \quad (1999)$$

$$\tau^3_{\gamma,\delta,w} = \sum_{\epsilon \in A} Z_{\epsilon,\gamma} \tau^2_{\epsilon,\delta,w} \quad (2r_D r_T^3) \quad (2000)$$

$$\tau^4_{\alpha,i} = \sum_{a \in V} {}^1T_{a,i} W^4_{a,\alpha} \quad (2r_V N_o N_v) \quad (2001)$$

$$\tau^5_{\alpha,\beta} = \sum_{i \in O} W^1_{i,\alpha} \tau^4_{\beta,i} \quad (2r_V^2 N_o) \quad (2002)$$



$$\tau_{\alpha,i}^6 = \sum_{\beta \in B} X_{\alpha,\beta} W_{i,\beta}^3 \tau_{\alpha,\beta}^5 \quad (3r_V^2 N_o) \quad (2003)$$

$$\tau_{\alpha,i,j}^6 = \sum_{\beta \in B} X_{\alpha,\beta} W_{j,\beta}^3 \tau_{\beta,i}^5 \quad (3r_V^2 N_o^2) \quad (2016)$$

$$\tau_{i,a}^7 = \sum_{\alpha \in B} W_{a,\alpha}^2 \tau_{\alpha,i}^6 \quad (2r_V N_o N_v) \quad (2004)$$

$$\tau_{\gamma,\alpha,i}^7 = \sum_{j \in O} Y_{j,\gamma}^4 \tau_{\alpha,i,j}^6 \quad (2r_T r_V N_o^2) \quad (2017)$$

$$\tau_{i,j}^8 = \sum_{a \in V} {}^1T_{a,i} \tau_{j,a}^7 \quad (2N_o^2 N_v) \quad (2005)$$

$$\tau_{\gamma,\delta,w,i}^8 = \sum_{\alpha \in B} \tau_{\gamma,\alpha,i}^7 \tau_{\gamma,\delta,\alpha,w}^4 \quad (2r_D r_T^2 r_V N_o) \quad (2018)$$

$$\tau_{\gamma,i}^9 = \sum_{j \in O} Y_{j,\gamma}^4 \tau_{i,j}^8 \quad (2r_T N_o^2) \quad (2006)$$

$$\tau_{\gamma,\delta,w}^9 = \sum_{\epsilon \in A} \sum_{i \in O} {}^2D_{i,w}^2 Y_{i,\delta}^{2,*} Z_{\delta,\epsilon}^* \tau_{\gamma,\epsilon,w,i}^8 \quad (4r_D r_T^3 N_o) \quad (2019)$$

$$\tau_{\gamma,\delta,w}^{10} = \sum_{i \in O} {}^2D_{i,w}^2 Y_{i,\delta}^{2,*} \tau_{\gamma,i}^9 \quad (3r_D r_T^2 N_o) \quad (2007)$$

$${}^{21}R_{a,\gamma} \leftarrow \sum_{\delta \in A} \sum_{w \in D} \frac{1}{2} {}^2D_{a,w}^1 Y_{a,\delta}^3 \tau_{\delta,\gamma,w}^9 \quad (3r_D r_T^2 N_v) \quad (2020)$$

$${}^{21}R_{a,\gamma} \leftarrow \sum_{\delta \in A} \sum_{w \in D} \frac{1}{2} {}^2D_{a,w}^1 Y_{a,\delta}^3 \tau_{\delta,\gamma,w}^{10} \tau_{\delta,\gamma,w}^3 \quad (4r_D r_T^2 N_v) \quad (2008)$$

Raw expression

$${}^{21}R_{a,\epsilon} \leftarrow - \sum_{\gamma \in A} \sum_{i \in O} \sum_{j \in O} \sum_{k \in O} \sum_{l \in O} \sum_{b \in V} \sum_{c \in V} \sum_{d \in V} {}^1T_{c,k} \\ {}^1T_{d,i} Y_{i,\epsilon}^{2,*} Z_{\epsilon,\gamma}^* Y_{b,\gamma}^{3,*} \\ Y_{j,\gamma}^{4,*} {}^2D_{a,i,b,j} {}^2T_{b,j,a,l} V_{k,c,l,d} \quad (2009)$$

Factorized expression

$$\tau_{\alpha,i}^0 = \sum_{a \in V} {}^1T_{a,i} W_{a,\alpha}^2 \quad (2r_V N_o N_v) \quad (2010)$$

$$\tau_{\gamma,\alpha,w}^1 = \sum_{i \in O} {}^2D_{i,w}^4 Y_{i,\gamma}^{4,*} \tau_{\alpha,i}^0 \quad (3r_D r_T r_V N_o) \quad (2011)$$

$$\tau_{\gamma,\delta,w}^2 = \sum_{a \in V} {}^2D_{a,w}^3 Y_{a,\gamma}^1 Y_{a,\delta}^{3,*} \quad (3r_D r_T^2 N_v) \quad (2012)$$

$$\tau_{\gamma,\delta,w,i}^3 = \sum_{\epsilon \in A} Y_{i,\epsilon}^2 Z_{\epsilon,\gamma} \tau_{\epsilon,\delta,w}^2 \quad (3r_D r_T^3 N_o) \quad (2013)$$

$$\tau_{\gamma,\delta,\alpha,w}^4 = \sum_{i \in O} W_{i,\alpha}^1 \tau_{\delta,\alpha,w}^1 \tau_{\gamma,\delta,w,i}^3 \quad (3r_D r_T^2 r_V N_o) \quad (2014)$$

$$\tau_{\alpha,i}^5 = \sum_{a \in V} {}^1T_{a,i} W_{a,\alpha}^4 \quad (2r_V N_o N_v) \quad (2015)$$

Raw expression

$${}^{21}R_{a,\epsilon} \leftarrow - \sum_{\gamma \in A} \sum_{i \in O} \sum_{j \in O} \sum_{k \in O} \sum_{l \in O} \sum_{b \in V} \sum_{c \in V} \sum_{d \in V} {}^1T_{c,k} \\ {}^1T_{d,j} Y_{i,\epsilon}^{2,*} Z_{\epsilon,\gamma}^* Y_{b,\gamma}^{3,*} \\ Y_{j,\gamma}^{4,*} {}^2D_{a,i,b,j} {}^2T_{a,i,b,l} V_{k,c,l,d} \quad (2021)$$

Factorized expression

$$\tau_{\gamma,\delta,w}^0 = \sum_{i \in O} {}^2D_{i,w}^2 Y_{i,\gamma}^2 Y_{i,\delta}^{2,*} \quad (3r_D r_T^2 N_o) \quad (2022)$$

$$\tau_{\gamma,\delta,w}^1 = \sum_{a \in V} {}^2D_{a,w}^3 Y_{a,\gamma}^3 Y_{a,\delta}^{3,*} \quad (3r_D r_T^2 N_v) \quad (2023)$$

$$\tau_{\alpha,i}^2 = \sum_{a \in V} {}^1T_{a,i} W_{a,\alpha}^4 \quad (2r_V N_o N_v) \quad (2024)$$

$$\tau_{\alpha,\beta}^3 = \sum_{i \in O} W_{i,\alpha}^1 \tau_{\beta,i}^2 \quad (2r_V^2 N_o) \quad (2025)$$

$$\tau_{\alpha,i}^4 = \sum_{\beta \in B} X_{\alpha,\beta} W_{i,\beta}^3 \tau_{\alpha,\beta}^3 \quad (3r_V^2 N_o) \quad (2026)$$

$$\tau_{i,a}^5 = \sum_{\alpha \in B} W_{a,\alpha}^2 \tau_{\alpha,i}^4 \quad (2r_V N_o N_v) \quad (2027)$$

$$\tau_{i,j}^6 = \sum_{a \in V} {}^1T_{a,i} \tau_{j,a}^5 \quad (2N_o^2 N_v) \quad (2028)$$

$$\tau^7_{\gamma,i} = \sum_{j \in O} Y^4_{j,\gamma} \tau^6_{i,j} \quad (2r_T N_o^2) \quad (2029)$$

$$\tau^7_{\gamma,i} = \sum_{j \in O} Y^2_{j,\gamma} \tau^6_{i,j} \quad (2r_T N_o^2) \quad (2042)$$

$$\tau^8_{\gamma,\delta,w} = \sum_{i \in O} {}^2D^4_{i,w} Y^{4,*}_{i,\delta} \tau^7_{\gamma,i} \quad (3r_D r_T^2 N_o) \quad (2030)$$

$$\tau^8_{\gamma,\delta,w} = \sum_{i \in O} {}^2D^4_{i,w} Y^{4,*}_{i,\delta} \tau^7_{\gamma,i} \quad (3r_D r_T^2 N_o) \quad (2043)$$

$$\tau^9_{\gamma,\delta,w} = \sum_{\epsilon \in A} Z^*_{\delta,\epsilon} \tau^1_{\gamma,\epsilon,w} \tau^8_{\gamma,\epsilon,w} \quad (3r_D r_T^3) \quad (2031)$$

$$\tau^9_{\gamma,\delta,w} = \sum_{\epsilon \in A} Z^*_{\delta,\epsilon} \tau^1_{\gamma,\epsilon,w} \tau^8_{\gamma,\epsilon,w} \quad (3r_D r_T^3) \quad (2044)$$

$$\tau^{10}_{\gamma,\delta,w} = \sum_{\epsilon \in A} Z_{\gamma,\epsilon} \tau^9_{\epsilon,\delta,w} \quad (2r_D r_T^3) \quad (2032)$$

$$\tau^{10}_{\gamma,\delta,w} = \sum_{\epsilon \in A} Z_{\epsilon,\gamma} \tau^9_{\epsilon,\delta,w} \quad (2r_D r_T^3) \quad (2045)$$

$${}^{21}R_{a,\gamma} \leftarrow \sum_{\delta \in A} \sum_{w \in D} \frac{1}{2} {}^2D^1_{a,w} Y^1_{a,\delta} \tau^0_{\delta,\gamma,w} \tau^{10}_{\delta,\gamma,w} \quad (4r_D r_T^2 N_v) \quad (2033)$$

$${}^{21}R_{a,\gamma} \leftarrow \sum_{\delta \in A} \sum_{w \in D} \frac{1}{2} {}^2D^1_{a,w} Y^3_{a,\delta} \tau^0_{\delta,\gamma,w} \tau^{10}_{\delta,\gamma,w} \quad (4r_D r_T^2 N_v) \quad (2046)$$

Raw expression

$${}^{21}R_{a,\epsilon} \leftarrow - \sum_{\gamma \in A} \sum_{i \in O} \sum_{j \in O} \sum_{k \in O} \sum_{l \in O} \sum_{b \in V} \sum_{c \in V} \sum_{d \in V} {}^1T_{c,k} \\ {}^1T_{d,j} Y^{2,*}_{i,\epsilon} Z^*_{\epsilon,\gamma} Y^{3,*}_{b,\gamma} Y^{4,*}_{j,\gamma} {}^2D^{a,i,b,j} {}^2T_{b,l,a,i} V_{k,c,l,d} \quad (2034)$$

Factorized expression

$$\tau^0_{\gamma,\delta,w} = \sum_{i \in O} {}^2D^2_{i,w} Y^4_{i,\gamma} Y^{2,*}_{i,\delta} \quad (3r_D r_T^2 N_o) \quad (2035)$$

$$\tau^1_{\gamma,\delta,w} = \sum_{a \in V} {}^2D^3_{a,w} Y^1_{a,\gamma} Y^{3,*}_{a,\delta} \quad (3r_D r_T^2 N_v) \quad (2036)$$

$$\tau^2_{\alpha,i} = \sum_{a \in V} {}^1T_{a,i} W^4_{a,\alpha} \quad (2r_V N_o N_v) \quad (2037)$$

$$\tau^3_{\alpha,\beta} = \sum_{i \in O} W^1_{i,\alpha} \tau^2_{\beta,i} \quad (2r_V^2 N_o) \quad (2038)$$

$$\tau^4_{\alpha,i} = \sum_{\beta \in B} X_{\alpha,\beta} W^3_{i,\beta} \tau^3_{\alpha,\beta} \quad (3r_V^2 N_o) \quad (2039)$$

$$\tau^5_{i,a} = \sum_{\alpha \in B} W^2_{a,\alpha} \tau^4_{\alpha,i} \quad (2r_V N_o N_v) \quad (2040)$$

$$\tau^6_{i,j} = \sum_{a \in V} {}^1T_{a,i} \tau^5_{j,a} \quad (2N_o^2 N_v) \quad (2041)$$

## I. Contributions from $(H^2 T^2 T)_c$

Raw expression

$${}^{21}R_{a,\epsilon} \leftarrow \sum_{\gamma \in A} \sum_{i \in O} \sum_{j \in O} \sum_{k \in O} \sum_{l \in O} \sum_{b \in V} \sum_{c \in V} \sum_{d \in V} Y^{2,*}_{i,\epsilon} Z^*_{\epsilon,\gamma} \\ Y^{3,*}_{b,\gamma} Y^{4,*}_{j,\gamma} {}^2D^{a,i,b,j} {}^2T_{a,i,c,k} {}^2T_{b,j,d,l} V_{k,c,l,d} \quad (2047)$$

Factorized expression

$$\tau^0_{\gamma,\delta,w} = \sum_{i \in O} {}^2D^2_{i,w} Y^2_{i,\gamma} Y^{2,*}_{i,\delta} \quad (3r_D r_T^2 N_o) \quad (2048)$$

$$\tau^1_{\gamma,\delta,w} = \sum_{a \in V} {}^2D^3_{a,w} Y^1_{a,\gamma} Y^{3,*}_{a,\delta} \quad (3r_D r_T^2 N_v) \quad (2049)$$

$$\tau^2_{\gamma,\delta,w} = \sum_{i \in O} {}^2D^4_{i,w} Y^2_{i,\gamma} Y^{4,*}_{i,\delta} \quad (3r_D r_T^2 N_o) \quad (2050)$$

$$\tau^3_{\gamma,\delta,w} = \sum_{\epsilon \in A} Z^*_{\delta,\epsilon} \tau^1_{\gamma,\epsilon,w} \tau^2_{\gamma,\epsilon,w} \quad (3r_D r_T^3) \quad (2051)$$

$$\tau^4_{\gamma,\alpha} = \sum_{a \in V} W^4_{a,\alpha} Y^3_{a,\gamma} \quad (2r_T r_V N_v) \quad (2052)$$

$$\tau^5_{\gamma,\alpha} = \sum_{i \in O} W^3_{i,\alpha} Y^4_{i,\gamma} \quad (2r_T r_V N_o) \quad (2053)$$

$$\tau^6_{\gamma,\alpha} = \sum_{\beta \in B} X_{\alpha,\beta} \tau^4_{\gamma,\beta} \tau^5_{\gamma,\beta} \quad (3r_T r_V^2) \quad (2054)$$

$$\tau^4_{\gamma,\alpha} = \sum_{a \in V} W^2_{a,\alpha} Y^3_{a,\gamma} \quad (2r_T r_V N_v) \quad (2067)$$

$$\tau^7_{\gamma,\alpha} = \sum_{a \in V} W^2_{a,\alpha} Y^3_{a,\gamma} \quad (2r_T r_V N_v) \quad (2055)$$

$$\tau^5_{\gamma,\alpha} = \sum_{i \in O} W^1_{i,\alpha} Y^4_{i,\gamma} \quad (2r_T r_V N_o) \quad (2068)$$

$$\tau^8_{\gamma,\alpha} = \sum_{i \in O} W^1_{i,\alpha} Y^4_{i,\gamma} \quad (2r_T r_V N_o) \quad (2056)$$

$$\tau^6_{\gamma,\alpha} = \sum_{a \in V} W^4_{a,\alpha} Y^1_{a,\gamma} \quad (2r_T r_V N_v) \quad (2069)$$

$$\tau^9_{\gamma,\delta} = \sum_{\alpha \in B} \tau^6_{\delta,\alpha} \tau^7_{\gamma,\alpha} \tau^8_{\gamma,\alpha} \quad (3r_T^2 r_V) \quad (2057)$$

$$\tau^7_{\gamma,\alpha} = \sum_{i \in O} W^3_{i,\alpha} Y^2_{i,\gamma} \quad (2r_T r_V N_o) \quad (2070)$$

$$\tau^{10}_{\gamma,\delta} = \sum_{\epsilon \in A} Z_{\gamma,\epsilon} \tau^9_{\delta,\epsilon} \quad (2r_T^3) \quad (2058)$$

$$\tau^8_{\gamma,\alpha} = \sum_{\beta \in B} X_{\alpha,\beta} \tau^6_{\gamma,\beta} \tau^7_{\gamma,\beta} \quad (3r_T r_V^2) \quad (2071)$$

$$\tau^{11}_{\gamma,\delta} = \sum_{\epsilon \in A} Z_{\gamma,\epsilon} \tau^{10}_{\delta,\epsilon} \quad (2r_T^3) \quad (2059)$$

$$\tau^9_{\gamma,\delta} = \sum_{\alpha \in B} \tau^4_{\delta,\alpha} \tau^5_{\delta,\alpha} \tau^8_{\gamma,\alpha} \quad (3r_T^2 r_V) \quad (2072)$$

$$\tau^{12}_{\gamma,\delta,w} = \sum_{\epsilon \in A} \tau^{11}_{\gamma,\epsilon} \tau^3_{\epsilon,\delta,w} \quad (2r_D r_T^3) \quad (2060)$$

$$\tau^{10}_{\gamma,\delta} = \sum_{\epsilon \in A} Z_{\delta,\epsilon} \tau^9_{\gamma,\epsilon} \quad (2r_T^3) \quad (2073)$$

$${}^{21}R_{a,\gamma} \leftarrow \sum_{\delta \in A} \sum_{w \in D} {}^2D^1_{a,w} Y^1_{a,\delta} \tau^0_{\delta,\gamma,w} \tau^{12}_{\delta,\gamma,w} \quad (4r_D r_T^2 N_v) \quad (2061)$$

$$\tau^{11}_{\gamma,\delta} = \sum_{\epsilon \in A} Z_{\epsilon,\delta} \tau^{10}_{\epsilon,\gamma} \quad (2r_T^3) \quad (2074)$$

Raw expression

$$\tau^{12}_{\gamma,\delta,w} = \sum_{\epsilon \in A} \tau^{11}_{\gamma,\epsilon} \tau^3_{\epsilon,\delta,w} \quad (2r_D r_T^3) \quad (2075)$$

$${}^{21}R_{a,\epsilon} \leftarrow \sum_{\gamma \in A} \sum_{i \in O} \sum_{j \in O} \sum_{k \in O} \sum_{l \in O} \sum_{b \in V} \sum_{c \in V} \sum_{d \in V} Y^{2,*}_{i,\epsilon} Z^*_{\epsilon,\gamma} Y^{3,*}_{b,\gamma} Y^{4,*}_{j,\gamma} {}^2D^{a,i,b,j} {}^2T_{a,i,c,k} {}^2T_{d,l,b,j} V_{k,c,l,d} \quad (2062)$$

$${}^{21}R_{a,\gamma} \leftarrow \sum_{\delta \in A} \sum_{w \in D} {}^2D^1_{a,w} Y^1_{a,\delta} \tau^0_{\delta,\gamma,w} \tau^{12}_{\delta,\gamma,w} \quad (4r_D r_T^2 N_v) \quad (2076)$$

Factorized expression

Raw expression

$$\tau^0_{\gamma,\delta,w} = \sum_{i \in O} {}^2D^2_{i,w} Y^2_{i,\gamma} Y^{2,*}_{i,\delta} \quad (3r_D r_T^2 N_o) \quad (2063)$$

$${}^{21}R_{a,\epsilon} \leftarrow \sum_{\gamma \in A} \sum_{i \in O} \sum_{j \in O} \sum_{k \in O} \sum_{l \in O} \sum_{b \in V} \sum_{c \in V} \sum_{d \in V} Y^{2,*}_{i,\epsilon} Z^*_{\epsilon,\gamma} Y^{3,*}_{b,\gamma} Y^{4,*}_{j,\gamma} {}^2D^{a,i,b,j} {}^2T_{b,j,d,l} {}^2T_{c,k,a,i} V_{k,c,l,d} \quad (2077)$$

$$\tau^1_{\gamma,\delta,w} = \sum_{a \in V} {}^2D^3_{a,w} Y^3_{a,\gamma} Y^{3,*}_{a,\delta} \quad (3r_D r_T^2 N_v) \quad (2064)$$

Factorized expression

$$\tau^2_{\gamma,\delta,w} = \sum_{i \in O} {}^2D^4_{i,w} Y^4_{i,\gamma} Y^{4,*}_{i,\delta} \quad (3r_D r_T^2 N_o) \quad (2065)$$

$$\tau^0_{\gamma,\delta,w} = \sum_{i \in O} {}^2D^2_{i,w} Y^4_{i,\gamma} Y^{2,*}_{i,\delta} \quad (3r_D r_T^2 N_o) \quad (2078)$$

$$\tau^3_{\gamma,\delta,w} = \sum_{\epsilon \in A} Z^*_{\delta,\epsilon} \tau^1_{\gamma,\epsilon,w} \tau^2_{\gamma,\epsilon,w} \quad (3r_D r_T^3) \quad (2066)$$

$$\tau^1_{\gamma,\delta,w} = \sum_{a \in V} {}^2D^3_{a,w} Y^1_{a,\gamma} Y^{3,*}_{a,\delta} \quad (3r_D r_T^2 N_v) \quad (2079)$$

$$\tau^2_{\gamma,\delta,w} = \sum_{i \in O} {}^2D^4_{i,w} Y^2_{i,\gamma} Y^{4,*}_{i,\delta} \quad (3r_D r_T^2 N_o) \quad (2080)$$

$$\tau^0_{\gamma,\delta,w} = \sum_{i \in O} {}^2D^2_{i,w} Y^4_{i,\gamma} Y^{2,*}_{i,\delta} \quad (3r_D r_T^2 N_o) \quad (2093)$$

$$\tau^3_{\gamma,\delta,w} = \sum_{\epsilon \in A} Z^*_{\delta,\epsilon} \tau^1_{\gamma,\epsilon,w} \tau^2_{\gamma,\epsilon,w} \quad (3r_D r_T^3) \quad (2081)$$

$$\tau^1_{\gamma,\delta,w} = \sum_{a \in V} {}^2D^3_{a,w} Y^3_{a,\gamma} Y^{3,*}_{a,\delta} \quad (3r_D r_T^2 N_v) \quad (2094)$$

$$\tau^4_{\gamma,\alpha} = \sum_{a \in V} W^4_{a,\alpha} Y^3_{a,\gamma} \quad (2r_T r_V N_v) \quad (2082)$$

$$\tau^2_{\gamma,\delta,w} = \sum_{i \in O} {}^2D^4_{i,w} Y^4_{i,\gamma} Y^{4,*}_{i,\delta} \quad (3r_D r_T^2 N_o) \quad (2095)$$

$$\tau^5_{\gamma,\alpha} = \sum_{i \in O} W^3_{i,\alpha} Y^4_{i,\gamma} \quad (2r_T r_V N_o) \quad (2083)$$

$$\tau^3_{\gamma,\delta,w} = \sum_{\epsilon \in A} Z^*_{\delta,\epsilon} \tau^1_{\gamma,\epsilon,w} \tau^2_{\gamma,\epsilon,w} \quad (3r_D r_T^3) \quad (2096)$$

$$\tau^6_{\gamma,\alpha} = \sum_{\beta \in B} X_{\alpha,\beta} \tau^4_{\gamma,\beta} \tau^5_{\gamma,\beta} \quad (3r_T r_V^2) \quad (2084)$$

$$\tau^4_{\gamma,\alpha} = \sum_{a \in V} W^4_{a,\alpha} Y^1_{a,\gamma} \quad (2r_T r_V N_v) \quad (2097)$$

$$\tau^7_{\gamma,\alpha} = \sum_{a \in V} W^2_{a,\alpha} Y^1_{a,\gamma} \quad (2r_T r_V N_v) \quad (2085)$$

$$\tau^5_{\gamma,\alpha} = \sum_{i \in O} W^3_{i,\alpha} Y^2_{i,\gamma} \quad (2r_T r_V N_o) \quad (2098)$$

$$\tau^8_{\gamma,\alpha} = \sum_{i \in O} W^1_{i,\alpha} Y^2_{i,\gamma} \quad (2r_T r_V N_o) \quad (2086)$$

$$\tau^6_{\gamma,\alpha} = \sum_{\beta \in B} X_{\alpha,\beta} \tau^4_{\gamma,\beta} \tau^5_{\gamma,\beta} \quad (3r_T r_V^2) \quad (2099)$$

$$\tau^9_{\gamma,\delta} = \sum_{\alpha \in B} \tau^6_{\delta,\alpha} \tau^7_{\gamma,\alpha} \tau^8_{\gamma,\alpha} \quad (3r_T^2 r_V) \quad (2087)$$

$$\tau^7_{\gamma,\alpha} = \sum_{a \in V} W^2_{a,\alpha} Y^1_{a,\gamma} \quad (2r_T r_V N_v) \quad (2100)$$

$$\tau^{10}_{\gamma,\delta} = \sum_{\epsilon \in A} Z_{\delta,\epsilon} \tau^9_{\gamma,\epsilon} \quad (2r_T^3) \quad (2088)$$

$$\tau^8_{\gamma,\alpha} = \sum_{i \in O} W^1_{i,\alpha} Y^2_{i,\gamma} \quad (2r_T r_V N_o) \quad (2101)$$

$$\tau^{11}_{\gamma,\delta} = \sum_{\epsilon \in A} Z_{\epsilon,\delta} \tau^{10}_{\epsilon,\gamma} \quad (2r_T^3) \quad (2089)$$

$$\tau^9_{\gamma,\delta} = \sum_{\alpha \in B} \tau^6_{\delta,\alpha} \tau^7_{\gamma,\alpha} \tau^8_{\gamma,\alpha} \quad (3r_T^2 r_V) \quad (2102)$$

$$\tau^{12}_{\gamma,\delta,w} = \sum_{\epsilon \in A} \tau^{11}_{\epsilon,\gamma} \tau^3_{\epsilon,\delta,w} \quad (2r_D r_T^3) \quad (2090)$$

$$\tau^{10}_{\gamma,\delta} = \sum_{\epsilon \in A} Z_{\epsilon,\delta} \tau^9_{\gamma,\epsilon} \quad (2r_T^3) \quad (2103)$$

$${}^{21}R_{a,\gamma} \leftarrow \sum_{\delta \in A} \sum_{w \in D} {}^2D^1_{a,w} Y^3_{a,\delta} \tau^0_{\delta,\gamma,w} \tau^{12}_{\delta,\gamma,w} \quad (4r_D r_T^2 N_v) \quad (2091)$$

$$\tau^{11}_{\gamma,\delta} = \sum_{\epsilon \in A} Z_{\epsilon,\gamma} \tau^{10}_{\epsilon,\delta} \quad (2r_T^3) \quad (2104)$$

Raw expression

$$\tau^{12}_{\gamma,\delta,w} = \sum_{\epsilon \in A} \tau^{11}_{\gamma,\epsilon} \tau^3_{\epsilon,\delta,w} \quad (2r_D r_T^3) \quad (2105)$$

$${}^{21}R_{a,\epsilon} \leftarrow \sum_{\gamma \in A} \sum_{i \in O} \sum_{j \in O} \sum_{k \in O} \sum_{l \in O} \sum_{b \in V} \sum_{c \in V} \sum_{d \in V} Y^{2,*}_{i,\epsilon} Z^*_{\epsilon,\gamma} Y^{3,*}_{b,\gamma} Y^{4,*}_{j,\gamma} {}^2D^{a,i,b,j}_{c,k,a,i} {}^2T_{c,k,a,i} {}^2T_{d,l,b,j} V_{k,c,l,d} \quad (2092)$$

$${}^{21}R_{a,\gamma} \leftarrow \sum_{\delta \in A} \sum_{w \in D} {}^2D^1_{a,w} Y^3_{a,\delta} \tau^0_{\delta,\gamma,w} \tau^{12}_{\delta,\gamma,w} \quad (4r_D r_T^2 N_v) \quad (2106)$$

Factorized expression

Raw expression

$${}^{21}R_{a,\epsilon} \leftarrow - \sum_{\gamma \in A} \sum_{i \in O} \sum_{j \in O} \sum_{k \in O} \sum_{l \in O} \sum_{b \in V} \sum_{c \in V} \sum_{d \in V} \frac{1}{2} \quad (2107)$$

$$Y^{2,*}_{i,\epsilon} Z^*_{\epsilon,\gamma} Y^{3,*}_{b,\gamma} Y^{4,*}_{j,\gamma} {}^2D^{a,i,b,j} {}^2T_{a,i,b,k} {}^2T_{c,j,d,l} V_{k,c,l,d}$$

Factorized expression

$$\tau^0_{\gamma,\delta,w} = \sum_{i \in O} {}^2D^2_{i,w} Y^2_{i,\gamma} Y^{2,*}_{i,\delta} \quad (3r_D r_T^2 N_o) \quad (2108)$$

$$\tau^1_{\gamma,\delta,w} = \sum_{a \in V} {}^2D^3_{a,w} Y^1_{a,\gamma} Y^{3,*}_{a,\delta} \quad (3r_D r_T^2 N_v) \quad (2109)$$

$$\tau^2_{\gamma,\delta,w} = \sum_{i \in O} {}^2D^4_{i,w} Y^2_{i,\gamma} Y^{4,*}_{i,\delta} \quad (3r_D r_T^2 N_o) \quad (2110)$$

$$\tau^3_{\gamma,\delta,w} = \sum_{\epsilon \in A} Z^*_{\delta,\epsilon} \tau^1_{\gamma,\epsilon,w} \tau^2_{\gamma,\epsilon,w} \quad (3r_D r_T^3) \quad (2111)$$

$$\tau^4_{\gamma,\alpha} = \sum_{a \in V} W^2_{a,\alpha} Y^3_{a,\gamma} \quad (2r_T r_V N_v) \quad (2112)$$

$$\tau^5_{\gamma,\alpha,i} = \sum_{\beta \in B} W^1_{i,\beta} X_{\beta,\alpha} \tau^4_{\gamma,\beta} \quad (3r_T r_V^2 N_o) \quad (2113)$$

$$\tau^6_{\gamma,\alpha} = \sum_{i \in O} W^3_{i,\alpha} Y^4_{i,\gamma} \quad (2r_T r_V N_o) \quad (2114)$$

$$\tau^7_{\gamma,\alpha} = \sum_{a \in V} W^4_{a,\alpha} Y^3_{a,\gamma} \quad (2r_T r_V N_v) \quad (2115)$$

$$\tau^8_{\gamma,\delta,i} = \sum_{\alpha \in B} \tau^6_{\gamma,\alpha} \tau^7_{\delta,\alpha} \tau^5_{\gamma,\alpha,i} \quad (3r_T^2 r_V N_o) \quad (2116)$$

$$\tau^9_{\gamma,\delta} = \sum_{i \in O} Y^4_{i,\delta} \tau^8_{\gamma,\delta,i} \quad (2r_T^2 N_o) \quad (2117)$$

$$\tau^{10}_{\gamma,\delta} = \sum_{\epsilon \in A} Z_{\gamma,\epsilon} \tau^9_{\delta,\epsilon} \quad (2r_T^3) \quad (2118)$$

$$\tau^{11}_{\gamma,\delta} = \sum_{\epsilon \in A} Z_{\gamma,\epsilon} \tau^{10}_{\delta,\epsilon} \quad (2r_T^3) \quad (2119)$$

$$\tau^{12}_{\gamma,\delta,w} = \sum_{\epsilon \in A} \tau^{11}_{\epsilon,\gamma} \tau^3_{\epsilon,\delta,w} \quad (2r_D r_T^3) \quad (2120)$$

$${}^{21}R_{a,\gamma} \leftarrow - \sum_{\delta \in A} \sum_{w \in D} \frac{1}{2} {}^2D^1_{a,w} Y^1_{a,\delta} \tau^0_{\delta,\gamma,w} \tau^{12}_{\delta,\gamma,w} \quad (4r_D r_T^2 N_v) \quad (2121)$$

Raw expression

$${}^{21}R_{a,\epsilon} \leftarrow - \sum_{\gamma \in A} \sum_{i \in O} \sum_{j \in O} \sum_{k \in O} \sum_{l \in O} \sum_{b \in V} \sum_{c \in V} \sum_{d \in V} \frac{1}{2} \quad (2122)$$

$$Y^{2,*}_{i,\epsilon} Z^*_{\epsilon,\gamma} Y^{3,*}_{b,\gamma} Y^{4,*}_{j,\gamma} {}^2D^{a,i,b,j} {}^2T_{a,i,b,k} {}^2T_{c,l,d,j} V_{k,d,l,c}$$

Factorized expression

$$\tau^0_{\gamma,\delta,w} = \sum_{i \in O} {}^2D^2_{i,w} Y^2_{i,\gamma} Y^{2,*}_{i,\delta} \quad (3r_D r_T^2 N_o) \quad (2123)$$

$$\tau^1_{\gamma,\alpha} = \sum_{i \in O} W^1_{i,\alpha} Y^2_{i,\gamma} \quad (2r_T r_V N_o) \quad (2124)$$

$$\tau^2_{\gamma,\alpha} = \sum_{a \in V} W^4_{a,\alpha} Y^3_{a,\gamma} \quad (2r_T r_V N_v) \quad (2125)$$

$$\tau^3_{\gamma,\alpha} = \sum_{i \in O} W^3_{i,\alpha} Y^4_{i,\gamma} \quad (2r_T r_V N_o) \quad (2126)$$

$$\tau^4_{\gamma,\alpha} = \sum_{\beta \in B} X_{\alpha,\beta} \tau^2_{\gamma,\beta} \tau^3_{\gamma,\beta} \quad (3r_T r_V^2) \quad (2127)$$

$$\tau^5_{\gamma,\alpha} = \sum_{\delta \in A} Z_{\gamma,\delta} \tau^4_{\delta,\alpha} \quad (2r_T^2 r_V) \quad (2128)$$

$$\tau^6_{\gamma,a} = \sum_{\alpha \in B} W^2_{a,\alpha} \tau^1_{\gamma,\alpha} \tau^5_{\gamma,\alpha} \quad (3r_T r_V N_v) \quad (2129)$$

$$\tau^7_{a,b} = \sum_{\gamma \in A} Y^1_{b,\gamma} \tau^6_{\gamma,a} \quad (2r_T N_v^2) \quad (2130)$$

$$\tau^8_{\gamma,a} = \sum_{b \in V} Y^3_{b,\gamma} \tau^7_{b,a} \quad (2r_T N_v^2) \quad (2131)$$

$$\tau^9_{\gamma,\delta,w} = \sum_{a \in V} {}^2D^3_{a,w} Y^{3,*}_{a,\delta} \tau^8_{\gamma,a} \quad (3r_D r_T^2 N_v) \quad (2132)$$

$$\tau^{10}_{\gamma,\delta,w} = \sum_{i \in O} {}^2D^4_{i,w} Y^4_{i,\gamma} Y^{4,*}_{i,\delta} \quad (3r_D r_T^2 N_o) \quad (2133)$$

$$\tau^{11}_{\gamma,\delta,w} = \sum_{\epsilon \in A} Z^*_{\delta,\epsilon} \tau^{10}_{\gamma,\epsilon,w} \tau^9_{\gamma,\epsilon,w} \quad (3r_D r_T^3) \quad (2134)$$

$$\tau^9_{\gamma,\delta,i} = \sum_{\epsilon \in A} Z_{\gamma,\epsilon} Y^4_{i,\epsilon} \tau^8_{\gamma,\delta,\epsilon} \quad (3r_T^3 N_o) \quad (2147)$$

$$\tau^{12}_{\gamma,\delta,w} = \sum_{\epsilon \in A} Z_{\gamma,\epsilon} \tau^{11}_{\epsilon,\delta,w} \quad (2r_D r_T^3) \quad (2135)$$

$$\tau^{10}_{\gamma,\delta,w} = \sum_{\epsilon \in A} \sum_{i \in O} {}^2D^4_{i,w} Y^{4,*}_{i,\delta} \tau^1_{\epsilon,\delta,w} \tau^9_{\epsilon,\gamma,i} \quad (4r_D r_T^3 N_o) \quad (2148)$$

$${}^{21}R_{a,\gamma} \leftarrow - \sum_{\delta \in A} \sum_{w \in D} \frac{1}{2} {}^2D^1_{a,w} Y^1_{a,\delta} \tau^0_{\delta,\gamma,w} \tau^{12}_{\delta,\gamma,w} \quad (4r_D r_T^2 N_v) \quad (2136)$$

$$\tau^{11}_{\gamma,\delta,w} = \sum_{\epsilon \in A} Z^*_{\delta,\epsilon} \tau^{10}_{\gamma,\epsilon,w} \quad (2r_D r_T^3) \quad (2149)$$

Raw expression

$${}^{21}R_{a,\epsilon} \leftarrow - \sum_{\gamma \in A} \sum_{i \in O} \sum_{j \in O} \sum_{k \in O} \sum_{l \in O} \sum_{b \in V} \sum_{c \in V} \sum_{d \in V} \frac{1}{2} \quad (2137)$$

$$Y^{2,*}_{i,\epsilon} \quad Z^*_{\epsilon,\gamma} \quad Y^{3,*}_{b,\gamma} \quad Y^{4,*}_{j,\gamma} \quad {}^2D^{a,i,b,j} \quad {}^2T_{a,i,c,j} \quad {}^2T_{b,k,d,l} \quad V_{k,c,l,d}$$

$${}^{21}R_{a,\gamma} \leftarrow - \sum_{\delta \in A} \sum_{w \in D} \frac{1}{2} {}^2D^1_{a,w} Y^1_{a,\delta} \tau^0_{\delta,\gamma,w} \tau^{11}_{\delta,\gamma,w} \quad (4r_D r_T^2 N_v) \quad (2150)$$

Raw expression

$${}^{21}R_{a,\epsilon} \leftarrow - \sum_{\gamma \in A} \sum_{i \in O} \sum_{j \in O} \sum_{k \in O} \sum_{l \in O} \sum_{b \in V} \sum_{c \in V} \sum_{d \in V} \frac{1}{2} \quad (2151)$$

$$Y^{2,*}_{i,\epsilon} \quad Z^*_{\epsilon,\gamma} \quad Y^{3,*}_{b,\gamma} \quad Y^{4,*}_{j,\gamma} \quad {}^2D^{a,i,b,j} \quad {}^2T_{a,i,c,j} \quad {}^2T_{d,k,b,l} \quad V_{k,d,l,c}$$

Factorized expression

$$\tau^0_{\gamma,\delta,w} = \sum_{i \in O} {}^2D^2_{i,w} Y^2_{i,\gamma} Y^{2,*}_{i,\delta} \quad (3r_D r_T^2 N_o) \quad (2138)$$

Factorized expression

$$\tau^0_{\gamma,\delta,w} = \sum_{a \in V} {}^2D^3_{a,w} Y^1_{a,\gamma} Y^{3,*}_{a,\delta} \quad (3r_D r_T^2 N_v) \quad (2152)$$

$$\tau^2_{\gamma,\alpha} = \sum_{a \in V} W^2_{a,\alpha} Y^3_{a,\gamma} \quad (2r_T r_V N_v) \quad (2140)$$

$$\tau^1_{\gamma,\delta,w} = \sum_{i \in O} {}^2D^4_{i,w} Y^2_{i,\gamma} Y^{4,*}_{i,\delta} \quad (3r_D r_T^2 N_o) \quad (2153)$$

$$\tau^3_{\gamma,\alpha} = \sum_{i \in O} W^1_{i,\alpha} Y^4_{i,\gamma} \quad (2r_T r_V N_o) \quad (2141)$$

$$\tau^2_{\gamma,\delta,w} = \sum_{\epsilon \in A} Z^*_{\delta,\epsilon} \tau^0_{\gamma,\epsilon,w} \tau^1_{\gamma,\epsilon,w} \quad (3r_D r_T^3) \quad (2154)$$

$$\tau^4_{\gamma,\alpha} = \sum_{\beta \in B} X_{\beta,\alpha} \tau^2_{\gamma,\beta} \tau^3_{\gamma,\beta} \quad (3r_T r_V^2) \quad (2142)$$

$$\tau^3_{\gamma,\delta,w} = \sum_{\epsilon \in A} Z_{\epsilon,\gamma} \tau^2_{\epsilon,\delta,w} \quad (2r_D r_T^3) \quad (2155)$$

$$\tau^5_{\gamma,\alpha} = \sum_{\delta \in A} Z_{\gamma,\delta} \tau^4_{\delta,\alpha} \quad (2r_T^2 r_V) \quad (2143)$$

$$\tau^4_{\gamma,\delta,w} = \sum_{i \in O} {}^2D^2_{i,w} Y^4_{i,\gamma} Y^{2,*}_{i,\delta} \quad (3r_D r_T^2 N_o) \quad (2156)$$

$$\tau^6_{\gamma,\alpha} = \sum_{a \in V} W^4_{a,\alpha} Y^3_{a,\gamma} \quad (2r_T r_V N_v) \quad (2144)$$

$$\tau^5_{\gamma,\alpha} = \sum_{i \in O} W^1_{i,\alpha} Y^2_{i,\gamma} \quad (2r_T r_V N_o) \quad (2157)$$

$$\tau^7_{\gamma,\delta,i} = \sum_{\alpha \in B} W^3_{i,\alpha} \tau^5_{\gamma,\alpha} \tau^6_{\delta,\alpha} \quad (3r_T^2 r_V N_o) \quad (2145)$$

$$\tau^6_{\gamma,\alpha} = \sum_{a \in V} W^4_{a,\alpha} Y^3_{a,\gamma} \quad (2r_T r_V N_v) \quad (2158)$$

$$\tau^8_{\gamma,\delta,\epsilon} = \sum_{i \in O} Y^2_{i,\gamma} \tau^7_{\delta,\epsilon,i} \quad (2r_T^3 N_o) \quad (2146)$$

$$\tau^7_{\gamma,\alpha} = \sum_{i \in O} W^3_{i,\alpha} Y^4_{i,\gamma} \quad (2r_T r_V N_o) \quad (2159)$$

$$\tau^8_{\gamma,\alpha} = \sum_{\beta \in B} X_{\alpha,\beta} \tau^6_{\gamma,\beta} \tau^7_{\gamma,\beta} \quad (3r_T r_V^2) \quad (2160)$$

$$\tau^6_{\gamma,\alpha} = \sum_{\delta \in A} Z_{\gamma,\delta} \tau^5_{\delta,\alpha} \quad (2r_T^2 r_V) \quad (2173)$$

$$\tau^9_{\gamma,\alpha} = \sum_{\delta \in A} Z_{\gamma,\delta} \tau^8_{\delta,\alpha} \quad (2r_T^2 r_V) \quad (2161)$$

$$\tau^7_{\gamma,\alpha} = \sum_{a \in V} W^2_{a,\alpha} Y^3_{a,\gamma} \quad (2r_T r_V N_v) \quad (2174)$$

$$\tau^{10}_{\gamma,a} = \sum_{\alpha \in B} W^2_{a,\alpha} \tau^5_{\gamma,\alpha} \tau^9_{\gamma,\alpha} \quad (3r_T r_V N_v) \quad (2162)$$

$$\tau^8_{\gamma,\delta,i} = \sum_{\alpha \in B} W^1_{i,\alpha} \tau^6_{\gamma,\alpha} \tau^7_{\delta,\alpha} \quad (3r_T^2 r_V N_o) \quad (2175)$$

$$\tau^{11}_{a,b} = \sum_{\gamma \in A} Y^1_{b,\gamma} \tau^{10}_{\gamma,a} \quad (2r_T N_v^2) \quad (2163)$$

$$\tau^9_{\gamma,\delta,\epsilon} = \sum_{i \in O} Y^2_{i,\gamma} Z_{\gamma,\epsilon} \tau^8_{\delta,\epsilon,i} \quad (3r_T^3 N_o) \quad (2176)$$

$$\tau^{12}_{\gamma,a} = \sum_{b \in V} Y^3_{b,\gamma} \tau^{11}_{b,a} \quad (2r_T N_v^2) \quad (2164)$$

$$\tau^{10}_{\gamma,\delta,i} = \sum_{\epsilon \in A} Y^4_{i,\epsilon} \tau^9_{\gamma,\delta,\epsilon} \quad (2r_T^3 N_o) \quad (2177)$$

$${}^{21}R_{a,\gamma} \leftarrow - \sum_{\delta \in A} \sum_{w \in D} \frac{1}{2} {}^2D^1_{a,w} \tau^{12}_{\delta,a} \tau^3_{\delta,\gamma,w} \tau^4_{\delta,\gamma,w} \quad (4r_D r_T^2 N_v) \quad (2165)$$

$$\tau^{11}_{\gamma,\delta,w} = \sum_{\epsilon \in A} \sum_{i \in O} {}^2D^2_{i,w} Y^{2,*}_{i,\delta} \tau^{10}_{\gamma,\epsilon,i} \tau^2_{\epsilon,\delta,w} \quad (4r_D r_T^3 N_o) \quad (2178)$$

Raw expression

$${}^{21}R_{a,\epsilon} \leftarrow - \sum_{\gamma \in A} \sum_{i \in O} \sum_{j \in O} \sum_{k \in O} \sum_{l \in O} \sum_{b \in V} \sum_{c \in V} \sum_{d \in V} \frac{1}{2} Y^{2,*}_{i,\epsilon} Z^*_{\epsilon,\gamma} Y^{3,*}_{b,\gamma} Y^{4,*}_{j,\gamma} {}^2D^{a,i,b,j} {}^2T_{a,i,c,k} {}^2T_{b,j,d,l} V_{k,d,l,c} \quad (2166)$$

Factorized expression

$$\tau^0_{\gamma,\delta,w} = \sum_{a \in V} {}^2D^3_{a,w} Y^1_{a,\gamma} Y^{3,*}_{a,\delta} \quad (3r_D r_T^2 N_v) \quad (2167)$$

$${}^{21}R_{a,\gamma} \leftarrow - \sum_{\delta \in A} \sum_{w \in D} \frac{1}{2} {}^2D^1_{a,w} Y^1_{a,\delta} \tau^{11}_{\delta,\gamma,w} \quad (3r_D r_T^2 N_v) \quad (2179)$$

Raw expression

$${}^{21}R_{a,\epsilon} \leftarrow - \sum_{\gamma \in A} \sum_{i \in O} \sum_{j \in O} \sum_{k \in O} \sum_{l \in O} \sum_{b \in V} \sum_{c \in V} \sum_{d \in V} \frac{1}{2} Y^{2,*}_{i,\epsilon} Z^*_{\epsilon,\gamma} Y^{3,*}_{b,\gamma} Y^{4,*}_{j,\gamma} {}^2D^{a,i,b,j} {}^2T_{a,i,c,k} {}^2T_{b,l,d,j} V_{k,c,l,d} \quad (2180)$$

Factorized expression

$$\tau^1_{\gamma,\delta,w} = \sum_{i \in O} {}^2D^4_{i,w} Y^2_{i,\gamma} Y^{4,*}_{i,\delta} \quad (3r_D r_T^2 N_o) \quad (2168)$$

$$\tau^0_{\gamma,\delta,w} = \sum_{i \in O} {}^2D^2_{i,w} Y^2_{i,\gamma} Y^{2,*}_{i,\delta} \quad (3r_D r_T^2 N_o) \quad (2181)$$

$$\tau^2_{\gamma,\delta,w} = \sum_{\epsilon \in A} Z^*_{\delta,\epsilon} \tau^0_{\gamma,\epsilon,w} \tau^1_{\gamma,\epsilon,w} \quad (3r_D r_T^3) \quad (2169)$$

$$\tau^1_{\gamma,\delta,w} = \sum_{a \in V} {}^2D^3_{a,w} Y^3_{a,\gamma} Y^{3,*}_{a,\delta} \quad (3r_D r_T^2 N_v) \quad (2182)$$

$$\tau^3_{\gamma,\alpha} = \sum_{a \in V} W^4_{a,\alpha} Y^3_{a,\gamma} \quad (2r_T r_V N_v) \quad (2170)$$

$$\tau^2_{\gamma,\alpha} = \sum_{a \in V} W^2_{a,\alpha} Y^1_{a,\gamma} \quad (2r_T r_V N_v) \quad (2183)$$

$$\tau^4_{\gamma,\alpha} = \sum_{i \in O} W^3_{i,\alpha} Y^4_{i,\gamma} \quad (2r_T r_V N_o) \quad (2171)$$

$$\tau^3_{\gamma,\alpha} = \sum_{a \in V} W^4_{a,\alpha} Y^3_{a,\gamma} \quad (2r_T r_V N_v) \quad (2184)$$

$$\tau^5_{\gamma,\alpha} = \sum_{\beta \in B} X_{\alpha,\beta} \tau^3_{\gamma,\beta} \tau^4_{\gamma,\beta} \quad (3r_T r_V^2) \quad (2172)$$

$$\tau^4_{\gamma,\alpha} = \sum_{i \in O} W^3_{i,\alpha} Y^4_{i,\gamma} \quad (2r_T r_V N_o) \quad (2185)$$

$$\tau^5_{\gamma,\alpha} = \sum_{\beta \in B} X_{\alpha,\beta} \tau^3_{\gamma,\beta} \tau^4_{\gamma,\beta} \quad (3r_T r_V^2) \quad (2186)$$

$$\tau^3_{\gamma,\alpha} = \sum_{\beta \in B} X_{\beta,\alpha} \tau^1_{\gamma,\beta} \tau^2_{\gamma,\beta} \quad (3r_T r_V^2) \quad (2199)$$

$$\tau^6_{\gamma,\alpha} = \sum_{\delta \in A} Z_{\gamma,\delta} \tau^5_{\delta,\alpha} \quad (2r_T^2 r_V) \quad (2187)$$

$$\tau^4_{\gamma,\alpha} = \sum_{\delta \in A} Z_{\delta,\gamma} \tau^3_{\delta,\alpha} \quad (2r_T^2 r_V) \quad (2200)$$

$$\tau^7_{\gamma,i} = \sum_{\alpha \in B} W^1_{i,\alpha} \tau^2_{\gamma,\alpha} \tau^6_{\gamma,\alpha} \quad (3r_T r_V N_o) \quad (2188)$$

$$\tau^5_{\gamma,\alpha} = \sum_{i \in O} W^3_{i,\alpha} Y^4_{i,\gamma} \quad (2r_T r_V N_o) \quad (2201)$$

$$\tau^8_{i,j} = \sum_{\gamma \in A} Y^2_{j,\gamma} \tau^7_{\gamma,i} \quad (2r_T N_o^2) \quad (2189)$$

$$\tau^6_{\gamma,a} = \sum_{\alpha \in B} W^4_{a,\alpha} \tau^4_{\gamma,\alpha} \tau^5_{\gamma,\alpha} \quad (3r_T r_V N_v) \quad (2202)$$

$$\tau^9_{\gamma,i} = \sum_{j \in O} Y^4_{j,\gamma} \tau^8_{j,i} \quad (2r_T N_o^2) \quad (2190)$$

$$\tau^7_{\gamma,\delta} = \sum_{a \in V} Y^3_{a,\delta} \tau^6_{\gamma,a} \quad (2r_T^2 N_v) \quad (2203)$$

$$\tau^{10}_{\gamma,\delta,w} = \sum_{i \in O} {}^2D^4_{i,w} Y^{4,*}_{i,\delta} \tau^9_{\gamma,i} \quad (3r_D r_T^2 N_o) \quad (2191)$$

$$\tau^8_{\gamma,a} = \sum_{\delta \in A} Y^3_{a,\delta} \tau^7_{\delta,\gamma} \quad (2r_T^2 N_v) \quad (2204)$$

$$\tau^{11}_{\gamma,\delta,w} = \sum_{\epsilon \in A} Z^*_{\delta,\epsilon} \tau^1_{\gamma,\epsilon,w} \tau^{10}_{\gamma,\epsilon,w} \quad (3r_D r_T^3) \quad (2192)$$

$$\tau^9_{\gamma,\delta,w} = \sum_{a \in V} {}^2D^3_{a,w} Y^{3,*}_{a,\delta} \tau^8_{\gamma,a} \quad (3r_D r_T^2 N_v) \quad (2205)$$

$$\tau^{12}_{\gamma,\delta,w} = \sum_{\epsilon \in A} Z_{\gamma,\epsilon} \tau^{11}_{\epsilon,\delta,w} \quad (2r_D r_T^3) \quad (2193)$$

$$\tau^{10}_{\gamma,\delta,w} = \sum_{i \in O} {}^2D^4_{i,w} Y^4_{i,\gamma} Y^{4,*}_{i,\delta} \quad (3r_D r_T^2 N_o) \quad (2206)$$

$${}^{21}R_{a,\gamma} \leftarrow - \sum_{\delta \in A} \sum_{w \in D} \frac{1}{2} {}^2D^1_{a,w} Y^1_{a,\delta} \tau^0_{\delta,\gamma,w} \tau^{12}_{\delta,\gamma,w} \quad (4r_D r_T^2 N_v) \quad (2194)$$

Raw expression

$$\tau^{12}_{\gamma,\delta,w} = \sum_{\epsilon \in A} Z_{\gamma,\epsilon} \tau^{11}_{\epsilon,\delta,w} \quad (2r_D r_T^3) \quad (2208)$$

$${}^{21}R_{a,\epsilon} \leftarrow - \sum_{\gamma \in A} \sum_{i \in O} \sum_{j \in O} \sum_{k \in O} \sum_{l \in O} \sum_{b \in V} \sum_{c \in V} \sum_{d \in V} \frac{1}{2} Y^{2,*}_{i,\epsilon} Z^*_{\epsilon,\gamma} Y^{3,*}_{b,\gamma} Y^{4,*}_{j,\gamma} {}^2D^{a,i,b,j} {}^2T_{a,i,c,k} {}^2T_{d,j,b,l} V_{k,c,l,d} \quad (2195)$$

$${}^{21}R_{a,\gamma} \leftarrow - \sum_{\delta \in A} \sum_{w \in D} \frac{1}{2} {}^2D^1_{a,w} Y^1_{a,\delta} \tau^0_{\delta,\gamma,w} \tau^{12}_{\delta,\gamma,w} \quad (4r_D r_T^2 N_v) \quad (2209)$$

Factorized expression

Raw expression

$$\tau^0_{\gamma,\delta,w} = \sum_{i \in O} {}^2D^2_{i,w} Y^2_{i,\gamma} Y^{2,*}_{i,\delta} \quad (3r_D r_T^2 N_o) \quad (2196)$$

$${}^{21}R_{a,\epsilon} \leftarrow - \sum_{\gamma \in A} \sum_{i \in O} \sum_{j \in O} \sum_{k \in O} \sum_{l \in O} \sum_{b \in V} \sum_{c \in V} \sum_{d \in V} \frac{1}{2} Y^{2,*}_{i,\epsilon} Z^*_{\epsilon,\gamma} Y^{3,*}_{b,\gamma} Y^{4,*}_{j,\gamma} {}^2D^{a,i,b,j} {}^2T_{a,i,c,k} {}^2T_{d,l,b,j} V_{k,d,l,c} \quad (2210)$$

$$\tau^1_{\gamma,\alpha} = \sum_{a \in V} W^2_{a,\alpha} Y^1_{a,\gamma} \quad (2r_T r_V N_v) \quad (2197)$$

Factorized expression

$$\tau^2_{\gamma,\alpha} = \sum_{i \in O} W^1_{i,\alpha} Y^2_{i,\gamma} \quad (2r_T r_V N_o) \quad (2198)$$

$$\tau^0_{\gamma,\delta,w} = \sum_{i \in O} {}^2D^2_{i,w} Y^2_{i,\gamma} Y^{2,*}_{i,\delta} \quad (3r_D r_T^2 N_o) \quad (2211)$$



$$\tau^1_{\gamma,\delta,w} = \sum_{a \in V} {}^2D^3_{a,w} Y^3_{a,\gamma} Y^{3,*}_{a,\delta} \quad (3r_D r_T^2 N_v) \quad (2212)$$

$$\tau^2_{\gamma,\delta,w} = \sum_{i \in O} {}^2D^4_{i,w} Y^4_{i,\gamma} Y^{4,*}_{i,\delta} \quad (3r_D r_T^2 N_o) \quad (2213)$$

$$\tau^3_{\gamma,\delta,w} = \sum_{\epsilon \in A} Z^*_{\delta,\epsilon} \tau^1_{\gamma,\epsilon,w} \tau^2_{\gamma,\epsilon,w} \quad (3r_D r_T^3) \quad (2214)$$

$$\tau^4_{\gamma,\alpha} = \sum_{a \in V} W^2_{a,\alpha} Y^1_{a,\gamma} \quad (2r_T r_V N_v) \quad (2215)$$

$$\tau^5_{\gamma,\alpha,i} = \sum_{\beta \in B} W^1_{i,\beta} X_{\beta,\alpha} \tau^4_{\gamma,\beta} \quad (3r_T r_V^2 N_o) \quad (2216)$$

$$\tau^6_{\gamma,\alpha} = \sum_{i \in O} W^3_{i,\alpha} Y^2_{i,\gamma} \quad (2r_T r_V N_o) \quad (2217)$$

$$\tau^7_{\gamma,\alpha} = \sum_{a \in V} W^4_{a,\alpha} Y^3_{a,\gamma} \quad (2r_T r_V N_v) \quad (2218)$$

$$\tau^8_{\gamma,\delta,i} = \sum_{\alpha \in B} \tau^6_{\gamma,\alpha} \tau^7_{\delta,\alpha} \tau^5_{\gamma,\alpha,i} \quad (3r_T^2 r_V N_o) \quad (2219)$$

$$\tau^9_{\gamma,\delta} = \sum_{i \in O} Y^4_{i,\delta} \tau^8_{\gamma,\delta,i} \quad (2r_T^2 N_o) \quad (2220)$$

$$\tau^{10}_{\gamma,\delta} = \sum_{\epsilon \in A} Z_{\delta,\epsilon} \tau^9_{\gamma,\epsilon} \quad (2r_T^3) \quad (2221)$$

$$\tau^{11}_{\gamma,\delta} = \sum_{\epsilon \in A} Z_{\epsilon,\delta} \tau^{10}_{\epsilon,\gamma} \quad (2r_T^3) \quad (2222)$$

$$\tau^{12}_{\gamma,\delta,w} = \sum_{\epsilon \in A} \tau^{11}_{\gamma,\epsilon} \tau^3_{\epsilon,\delta,w} \quad (2r_D r_T^3) \quad (2223)$$

$${}^{21}R_{a,\gamma} \leftarrow - \sum_{\delta \in A} \sum_{w \in D} \frac{1}{2} {}^2D^1_{a,w} Y^1_{a,\delta} \tau^0_{\delta,\gamma,w} \tau^{12}_{\delta,\gamma,w} \quad (4r_D r_T^2 N_v) \quad (2224)$$

Raw expression

$${}^{21}R_{a,\epsilon} \leftarrow - \sum_{\gamma \in A} \sum_{i \in O} \sum_{j \in O} \sum_{k \in O} \sum_{l \in O} \sum_{b \in V} \sum_{c \in V} \sum_{d \in V} \frac{1}{2} \quad (2225)$$

$$Y^{2,*}_{i,\epsilon} Z^*_{\epsilon,\gamma} Y^{3,*}_{b,\gamma} Y^{4,*}_{j,\gamma} {}^2D^{a,i,b,j} {}^2T_{a,k,b,j} {}^2T_{c,i,d,l} V_{k,c,l,d}$$

Factorized expression

$$\tau^0_{\gamma,\delta,w} = \sum_{i \in O} {}^2D^2_{i,w} Y^2_{i,\gamma} Y^{2,*}_{i,\delta} \quad (3r_D r_T^2 N_o) \quad (2226)$$

$$\tau^1_{\gamma,\delta,w} = \sum_{a \in V} {}^2D^3_{a,w} Y^3_{a,\gamma} Y^{3,*}_{a,\delta} \quad (3r_D r_T^2 N_v) \quad (2227)$$

$$\tau^2_{\gamma,\delta,w} = \sum_{i \in O} {}^2D^4_{i,w} Y^4_{i,\gamma} Y^{4,*}_{i,\delta} \quad (3r_D r_T^2 N_o) \quad (2228)$$

$$\tau^3_{\gamma,\delta,w} = \sum_{\epsilon \in A} Z^*_{\delta,\epsilon} \tau^1_{\gamma,\epsilon,w} \tau^2_{\gamma,\epsilon,w} \quad (3r_D r_T^3) \quad (2229)$$

$$\tau^4_{\gamma,\delta,w} = \sum_{\epsilon \in A} Z_{\gamma,\epsilon} \tau^3_{\epsilon,\delta,w} \quad (2r_D r_T^3) \quad (2230)$$

$$\tau^5_{\gamma,\alpha} = \sum_{i \in O} W^1_{i,\alpha} Y^2_{i,\gamma} \quad (2r_T r_V N_o) \quad (2231)$$

$$\tau^6_{\gamma,\alpha} = \sum_{a \in V} W^4_{a,\alpha} Y^3_{a,\gamma} \quad (2r_T r_V N_v) \quad (2232)$$

$$\tau^7_{\gamma,\alpha} = \sum_{i \in O} W^3_{i,\alpha} Y^4_{i,\gamma} \quad (2r_T r_V N_o) \quad (2233)$$

$$\tau^8_{\gamma,\alpha} = \sum_{\beta \in B} X_{\alpha,\beta} \tau^6_{\gamma,\beta} \tau^7_{\gamma,\beta} \quad (3r_T r_V^2) \quad (2234)$$

$$\tau^9_{\gamma,\alpha} = \sum_{\delta \in A} Z_{\gamma,\delta} \tau^8_{\delta,\alpha} \quad (2r_T^2 r_V) \quad (2235)$$

$$\tau^{10}_{\gamma,a} = \sum_{\alpha \in B} W^2_{a,\alpha} \tau^5_{\gamma,\alpha} \tau^9_{\gamma,\alpha} \quad (3r_T r_V N_v) \quad (2236)$$

$$\tau^{11}_{a,b} = \sum_{\gamma \in A} Y^1_{b,\gamma} \tau^{10}_{\gamma,a} \quad (2r_T N_v^2) \quad (2237)$$

$$\tau^{12}_{\gamma,a} = \sum_{b \in V} Y^1_{b,\gamma} \tau^{11}_{b,a} \quad (2r_T N_v^2) \quad (2238)$$

$${}^{21}R_{a,\gamma} \leftarrow - \sum_{\delta \in A} \sum_{w \in D} \frac{1}{2} {}^2D^1_{a,w} \tau^{12}_{\delta,a} \tau^0_{\delta,\gamma,w} \tau^4_{\delta,\gamma,w} \quad (4r_D r_T^2 N_v) \quad (2239)$$

Raw expression

$${}^{21}R_{a,\epsilon} \leftarrow - \sum_{\gamma \in A} \sum_{i \in O} \sum_{j \in O} \sum_{k \in O} \sum_{l \in O} \sum_{b \in V} \sum_{c \in V} \sum_{d \in V} \frac{1}{2} \quad (2240)$$

$$Y^{2,*}_{i,\epsilon} Z^*_{\epsilon,\gamma} Y^{3,*}_{b,\gamma} Y^{4,*}_{j,\gamma}$$

$${}^2D^{a,i,b,j} {}^2T_{a,k,b,j} {}^2T_{c,l,d,i} V_{k,d,l,c}$$

Factorized expression

$$\tau^0_{\gamma,\alpha} = \sum_{a \in V} W^2_{a,\alpha} Y^1_{a,\gamma} \quad (2r_T r_V N_v) \quad (2241)$$

$$\tau^1_{\gamma,\alpha} = \sum_{a \in V} W^4_{a,\alpha} Y^3_{a,\gamma} \quad (2r_T r_V N_v) \quad (2242)$$

$$\tau^2_{\gamma,\alpha} = \sum_{i \in O} W^3_{i,\alpha} Y^4_{i,\gamma} \quad (2r_T r_V N_o) \quad (2243)$$

$$\tau^3_{\gamma,\alpha} = \sum_{\beta \in B} X_{\alpha,\beta} \tau^1_{\gamma,\beta} \tau^2_{\gamma,\beta} \quad (3r_T r_V^2) \quad (2244)$$

$$\tau^4_{\gamma,\alpha} = \sum_{\delta \in A} Z_{\gamma,\delta} \tau^3_{\delta,\alpha} \quad (2r_T^2 r_V) \quad (2245)$$

$$\tau^5_{\gamma,i} = \sum_{\alpha \in B} W^1_{i,\alpha} \tau^0_{\gamma,\alpha} \tau^4_{\gamma,\alpha} \quad (3r_T r_V N_o) \quad (2246)$$

$$\tau^6_{i,j} = \sum_{\gamma \in A} Y^2_{j,\gamma} \tau^5_{\gamma,i} \quad (2r_T N_o^2) \quad (2247)$$

$$\tau^7_{\gamma,i} = \sum_{j \in O} Y^2_{j,\gamma} \tau^6_{j,i} \quad (2r_T N_o^2) \quad (2248)$$

$$\tau^8_{\gamma,\delta,w} = \sum_{i \in O} {}^2D^2_{i,w} Y^{2,*}_{i,\delta} \tau^7_{\gamma,i} \quad (3r_D r_T^2 N_o) \quad (2249)$$

$$\tau^9_{\gamma,\delta,w} = \sum_{a \in V} {}^2D^3_{a,w} Y^3_{a,\gamma} Y^{3,*}_{a,\delta} \quad (3r_D r_T^2 N_v) \quad (2250)$$

$$\tau^{10}_{\gamma,\delta,w} = \sum_{i \in O} {}^2D^4_{i,w} Y^4_{i,\gamma} Y^{4,*}_{i,\delta} \quad (3r_D r_T^2 N_o) \quad (2251)$$

$$\tau^{11}_{\gamma,\delta,w} = \sum_{\epsilon \in A} Z^*_{\delta,\epsilon} \tau^{10}_{\gamma,\epsilon,w} \tau^9_{\gamma,\epsilon,w} \quad (3r_D r_T^3) \quad (2252)$$

$$\tau^{12}_{\gamma,\delta,w} = \sum_{\epsilon \in A} Z_{\gamma,\epsilon} \tau^{11}_{\epsilon,\delta,w} \quad (2r_D r_T^3) \quad (2253)$$

$${}^{21}R_{a,\gamma} \leftarrow - \sum_{\delta \in A} \sum_{w \in D} \frac{1}{2} {}^2D^1_{a,w} Y^1_{a,\delta} \tau^{12}_{\delta,\gamma,w} \tau^8_{\delta,\gamma,w} \quad (4r_D r_T^2 N_v) \quad (2254)$$

Raw expression

$${}^{21}R_{a,\epsilon} \leftarrow - \sum_{\gamma \in A} \sum_{i \in O} \sum_{j \in O} \sum_{k \in O} \sum_{l \in O} \sum_{b \in V} \sum_{c \in V} \sum_{d \in V} \frac{1}{2} \quad (2255)$$

$$Y^{2,*}_{i,\epsilon} Z^*_{\epsilon,\gamma} Y^{3,*}_{b,\gamma} Y^{4,*}_{j,\gamma}$$

$${}^2D^{a,i,b,j} {}^2T_{a,k,c,i} {}^2T_{b,j,d,l} V_{k,c,l,d}$$

Factorized expression

$$\tau^0_{\gamma,\delta,w} = \sum_{i \in O} {}^2D^2_{i,w} Y^2_{i,\gamma} Y^{2,*}_{i,\delta} \quad (3r_D r_T^2 N_o) \quad (2256)$$

$$\tau^1_{\gamma,\delta,w} = \sum_{a \in V} {}^2D^3_{a,w} Y^3_{a,\gamma} Y^{3,*}_{a,\delta} \quad (3r_D r_T^2 N_v) \quad (2257)$$

$$\tau^2_{\gamma,\alpha} = \sum_{a \in V} W^4_{a,\alpha} Y^1_{a,\gamma} \quad (2r_T r_V N_v) \quad (2258)$$

$$\tau^3_{\gamma,\alpha} = \sum_{a \in V} W^2_{a,\alpha} Y^3_{a,\gamma} \quad (2r_T r_V N_v) \quad (2259)$$

$$\tau^4_{\gamma,\alpha} = \sum_{i \in O} W^1_{i,\alpha} Y^4_{i,\gamma} \quad (2r_T r_V N_o) \quad (2260)$$

$$\tau^5_{\gamma,\alpha} = \sum_{\beta \in B} X_{\beta,\alpha} \tau^3_{\gamma,\beta} \tau^4_{\gamma,\beta} \quad (3r_T r_V^2) \quad (2261)$$

$$\tau^6_{\gamma,\alpha} = \sum_{\delta \in A} Z_{\gamma,\delta} \tau^5_{\delta,\alpha} \quad (2r_T^2 r_V) \quad (2262)$$

$$\tau^7_{\gamma,\delta,i} = \sum_{\alpha \in B} W^3_{i,\alpha} \tau^2_{\gamma,\alpha} \tau^6_{\delta,\alpha} \quad (3r_T^2 r_V N_o) \quad (2263)$$

$$\tau^8_{\gamma,\delta,\epsilon} = \sum_{i \in O} Z_{\gamma,\epsilon} Y^4_{i,\epsilon} \tau^7_{\gamma,\delta,i} \quad (3r_T^3 N_o) \quad (2264)$$

$$\tau^9_{\gamma,\delta,i} = \sum_{\epsilon \in A} Y^2_{i,\epsilon} \tau^8_{\epsilon,\gamma,\delta} \quad (2r_T^3 N_o) \quad (2265)$$

$$\tau^{10}_{\gamma,\delta,w} = \sum_{\epsilon \in A} \sum_{i \in O} {}^2D^4_{i,w} Y^{4,*}_{i,\delta} \tau^1_{\epsilon,\delta,w} \tau^9_{\gamma,\epsilon,i} \quad (4r_D r_T^3 N_o) \quad (2266)$$

$$\tau^{11}_{\gamma,\delta,w} = \sum_{\epsilon \in A} Z^*_{\delta,\epsilon} \tau^{10}_{\gamma,\epsilon,w} \quad (2r_D r_T^3) \quad (2267)$$

$$\tau^{10}_{\gamma,\delta,w} = \sum_{i \in O} {}^2D^4_{i,w} Y^{4,*}_{i,\delta} \tau^9_{\gamma,i} \quad (3r_D r_T^2 N_o) \quad (2280)$$

$${}^{21}R_{a,\gamma} \leftarrow - \sum_{\delta \in A} \sum_{w \in D} \frac{1}{2} {}^2D^1_{a,w} Y^1_{a,\delta} \tau^0_{\delta,\gamma,w} \tau^{11}_{\delta,\gamma,w} \quad (4r_D r_T^2 N_v) \quad (2268)$$

$$\tau^{11}_{\gamma,\delta,w} = \sum_{\epsilon \in A} Z^*_{\delta,\epsilon} \tau^1_{\gamma,\epsilon,w} \tau^{10}_{\gamma,\epsilon,w} \quad (3r_D r_T^3) \quad (2281)$$

Raw expression

$$\tau^{12}_{\gamma,\delta,w} = \sum_{\epsilon \in A} Z_{\gamma,\epsilon} \tau^{11}_{\epsilon,\delta,w} \quad (2r_D r_T^3) \quad (2282)$$

$${}^{21}R_{a,\epsilon} \leftarrow - \sum_{\gamma \in A} \sum_{i \in O} \sum_{j \in O} \sum_{k \in O} \sum_{l \in O} \sum_{b \in V} \sum_{c \in V} \sum_{d \in V} \frac{1}{2} \quad (2269)$$

$$Y^{2,*}_{i,\epsilon} Z^*_{\epsilon,\gamma} Y^{3,*}_{b,\gamma} Y^{4,*}_{j,\gamma} {}^2D^{a,i,b,j} {}^2T_{a,k,c,i} {}^2T_{d,l,b,j} V_{k,c,l,d}$$

$${}^{21}R_{a,\gamma} \leftarrow - \sum_{\delta \in A} \sum_{w \in D} \frac{1}{2} {}^2D^1_{a,w} Y^1_{a,\delta} \tau^0_{\delta,\gamma,w} \tau^{12}_{\delta,\gamma,w} \quad (4r_D r_T^2 N_v) \quad (2283)$$

Factorized expression

Raw expression

$$\tau^0_{\gamma,\delta,w} = \sum_{i \in O} {}^2D^2_{i,w} Y^2_{i,\gamma} Y^{2,*}_{i,\delta} \quad (3r_D r_T^2 N_o) \quad (2270)$$

$${}^{21}R_{a,\epsilon} \leftarrow - \sum_{\gamma \in A} \sum_{i \in O} \sum_{j \in O} \sum_{k \in O} \sum_{l \in O} \sum_{b \in V} \sum_{c \in V} \sum_{d \in V} \frac{1}{2} \quad (2284)$$

$$Y^{2,*}_{i,\epsilon} Z^*_{\epsilon,\gamma} Y^{3,*}_{b,\gamma} Y^{4,*}_{j,\gamma} {}^2D^{a,i,b,j} {}^2T_{a,k,c,l} {}^2T_{b,j,d,i} V_{k,d,l,c}$$

$$\tau^1_{\gamma,\delta,w} = \sum_{a \in V} {}^2D^3_{a,w} Y^3_{a,\gamma} Y^{3,*}_{a,\delta} \quad (3r_D r_T^2 N_v) \quad (2271)$$

Factorized expression

$$\tau^2_{\gamma,\alpha} = \sum_{a \in V} W^4_{a,\alpha} Y^1_{a,\gamma} \quad (2r_T r_V N_v) \quad (2272)$$

$$\tau^0_{\gamma,\delta,w} = \sum_{a \in V} {}^2D^3_{a,w} Y^3_{a,\gamma} Y^{3,*}_{a,\delta} \quad (3r_D r_T^2 N_v) \quad (2285)$$

$$\tau^3_{\gamma,\alpha} = \sum_{i \in O} W^3_{i,\alpha} Y^2_{i,\gamma} \quad (2r_T r_V N_o) \quad (2273)$$

$$\tau^1_{\gamma,\delta,w} = \sum_{i \in O} {}^2D^4_{i,w} Y^4_{i,\gamma} Y^{4,*}_{i,\delta} \quad (3r_D r_T^2 N_o) \quad (2286)$$

$$\tau^4_{\gamma,\alpha} = \sum_{\beta \in B} X_{\alpha,\beta} \tau^2_{\gamma,\beta} \tau^3_{\gamma,\beta} \quad (3r_T r_V^2) \quad (2274)$$

$$\tau^2_{\gamma,\delta,w} = \sum_{\epsilon \in A} Z^*_{\delta,\epsilon} \tau^0_{\gamma,\epsilon,w} \tau^1_{\gamma,\epsilon,w} \quad (3r_D r_T^3) \quad (2287)$$

$$\tau^5_{\gamma,\alpha} = \sum_{\delta \in A} Z_{\delta,\gamma} \tau^4_{\delta,\alpha} \quad (2r_T^2 r_V) \quad (2275)$$

$$\tau^3_{\gamma,\alpha} = \sum_{a \in V} W^2_{a,\alpha} Y^3_{a,\gamma} \quad (2r_T r_V N_v) \quad (2288)$$

$$\tau^6_{\gamma,\alpha} = \sum_{a \in V} W^2_{a,\alpha} Y^3_{a,\gamma} \quad (2r_T r_V N_v) \quad (2276)$$

$$\tau^4_{\gamma,\alpha} = \sum_{a \in V} W^4_{a,\alpha} Y^1_{a,\gamma} \quad (2r_T r_V N_v) \quad (2289)$$

$$\tau^7_{\gamma,i} = \sum_{\alpha \in B} W^1_{i,\alpha} \tau^5_{\gamma,\alpha} \tau^6_{\gamma,\alpha} \quad (3r_T r_V N_o) \quad (2277)$$

$$\tau^5_{\gamma,\alpha} = \sum_{i \in O} W^3_{i,\alpha} Y^2_{i,\gamma} \quad (2r_T r_V N_o) \quad (2290)$$

$$\tau^8_{i,j} = \sum_{\gamma \in A} Y^4_{j,\gamma} \tau^7_{\gamma,i} \quad (2r_T N_o^2) \quad (2278)$$

$$\tau^6_{\gamma,\alpha} = \sum_{\beta \in B} X_{\alpha,\beta} \tau^4_{\gamma,\beta} \tau^5_{\gamma,\beta} \quad (3r_T r_V^2) \quad (2291)$$

$$\tau^9_{\gamma,i} = \sum_{j \in O} Y^4_{j,\gamma} \tau^8_{j,i} \quad (2r_T N_o^2) \quad (2279)$$

$$\tau^7_{\gamma,\alpha} = \sum_{\delta \in A} Z_{\delta,\gamma} \tau^6_{\delta,\alpha} \quad (2r_T^2 r_V) \quad (2292)$$

$$\tau^8_{\gamma,\delta,i} = \sum_{\alpha \in B} W^1_{i,\alpha} \tau^3_{\delta,\alpha} \tau^7_{\gamma,\alpha} \quad (3r_T^2 r_V N_o) \quad (2293)$$

$$\tau^7_{\gamma,i} = \sum_{j \in O} Y^2_{j,\gamma} \tau^6_{j,i} \quad (2r_T N_o^2) \quad (2306)$$

$$\tau^9_{\gamma,\delta,\epsilon} = \sum_{i \in O} Y^2_{i,\gamma} \tau^8_{\delta,\epsilon,i} \quad (2r_T^3 N_o) \quad (2294)$$

$$\tau^8_{\gamma,\delta,w} = \sum_{i \in O} {}^2D^2_{i,w} Y^{2,*}_{i,\delta} \tau^7_{\gamma,i} \quad (3r_D r_T^2 N_o) \quad (2307)$$

$$\tau^{10}_{\gamma,\delta,i} = \sum_{\epsilon \in A} Z_{\gamma,\epsilon} Y^4_{i,\epsilon} \tau^9_{\gamma,\delta,\epsilon} \quad (3r_T^3 N_o) \quad (2295)$$

$$\tau^9_{\gamma,\delta,w} = \sum_{a \in V} {}^2D^3_{a,w} Y^3_{a,\gamma} Y^{3,*}_{a,\delta} \quad (3r_D r_T^2 N_v) \quad (2308)$$

$$\tau^{11}_{\gamma,\delta,w} = \sum_{\epsilon \in A} \sum_{i \in O} {}^2D^2_{i,w} Y^{2,*}_{i,\delta} \tau^{10}_{\gamma,\epsilon,i} \tau^2_{\epsilon,\delta,w} \quad (4r_D r_T^3 N_o) \quad (2296)$$

$$\tau^{10}_{\gamma,\delta,w} = \sum_{i \in O} {}^2D^4_{i,w} Y^4_{i,\gamma} Y^{4,*}_{i,\delta} \quad (3r_D r_T^2 N_o) \quad (2309)$$

$${}^{21}R_{a,\gamma} \leftarrow - \sum_{\delta \in A} \sum_{w \in D} \frac{1}{2} {}^2D^1_{a,w} Y^1_{a,\delta} \tau^{11}_{\delta,\gamma,w} \quad (3r_D r_T^2 N_v) \quad (2297)$$

$$\tau^{11}_{\gamma,\delta,w} = \sum_{\epsilon \in A} Z^*_{\delta,\epsilon} \tau^{10}_{\gamma,\epsilon,w} \tau^9_{\gamma,\epsilon,w} \quad (3r_D r_T^3) \quad (2310)$$

Raw expression

$$\tau^{12}_{\gamma,\delta,w} = \sum_{\epsilon \in A} Z_{\gamma,\epsilon} \tau^{11}_{\epsilon,\delta,w} \quad (2r_D r_T^3) \quad (2311)$$

$${}^{21}R_{a,\epsilon} \leftarrow - \sum_{\gamma \in A} \sum_{i \in O} \sum_{j \in O} \sum_{k \in O} \sum_{l \in O} \sum_{b \in V} \sum_{c \in V} \sum_{d \in V} \frac{1}{2} \quad (2298)$$

$$Y^{2,*}_{i,\epsilon} Z^*_{\epsilon,\gamma} Y^{3,*}_{b,\gamma} Y^{4,*}_{j,\gamma} {}^2D^{a,i,b,j} {}^2T_{a,k,c,l} {}^2T_{d,i,b,j} V_{k,d,l,c}$$

$${}^{21}R_{a,\gamma} \leftarrow - \sum_{\delta \in A} \sum_{w \in D} \frac{1}{2} {}^2D^1_{a,w} Y^1_{a,\delta} \tau^{12}_{\delta,\gamma,w} \tau^8_{\delta,\gamma,w} \quad (4r_D r_T^2 N_v) \quad (2312)$$

Factorized expression

Raw expression

$$\tau^0_{\gamma,\alpha} = \sum_{a \in V} W^4_{a,\alpha} Y^1_{a,\gamma} \quad (2r_T r_V N_v) \quad (2299)$$

$${}^{21}R_{a,\epsilon} \leftarrow - \sum_{\gamma \in A} \sum_{i \in O} \sum_{j \in O} \sum_{k \in O} \sum_{l \in O} \sum_{b \in V} \sum_{c \in V} \sum_{d \in V} \frac{1}{2} \quad (2313)$$

$$Y^{2,*}_{i,\epsilon} Z^*_{\epsilon,\gamma} Y^{3,*}_{b,\gamma} Y^{4,*}_{j,\gamma} {}^2D^{a,i,b,j} {}^2T_{b,j,a,k} {}^2T_{c,i,d,l} V_{k,c,l,d}$$

$$\tau^1_{\gamma,\alpha} = \sum_{i \in O} W^3_{i,\alpha} Y^2_{i,\gamma} \quad (2r_T r_V N_o) \quad (2300)$$

Factorized expression

$$\tau^2_{\gamma,\alpha} = \sum_{\beta \in B} X_{\alpha,\beta} \tau^0_{\gamma,\beta} \tau^1_{\gamma,\beta} \quad (3r_T r_V^2) \quad (2301)$$

$$\tau^0_{\gamma,\alpha} = \sum_{a \in V} W^2_{a,\alpha} Y^1_{a,\gamma} \quad (2r_T r_V N_v) \quad (2314)$$

$$\tau^3_{\gamma,\alpha} = \sum_{\delta \in A} Z_{\delta,\gamma} \tau^2_{\delta,\alpha} \quad (2r_T^2 r_V) \quad (2302)$$

$$\tau^1_{\gamma,\alpha} = \sum_{a \in V} W^4_{a,\alpha} Y^3_{a,\gamma} \quad (2r_T r_V N_v) \quad (2315)$$

$$\tau^4_{\gamma,\alpha} = \sum_{a \in V} W^2_{a,\alpha} Y^3_{a,\gamma} \quad (2r_T r_V N_v) \quad (2303)$$

$$\tau^2_{\gamma,\alpha} = \sum_{i \in O} W^3_{i,\alpha} Y^4_{i,\gamma} \quad (2r_T r_V N_o) \quad (2316)$$

$$\tau^5_{\gamma,i} = \sum_{\alpha \in B} W^1_{i,\alpha} \tau^3_{\gamma,\alpha} \tau^4_{\gamma,\alpha} \quad (3r_T r_V N_o) \quad (2304)$$

$$\tau^3_{\gamma,\alpha} = \sum_{\beta \in B} X_{\alpha,\beta} \tau^1_{\gamma,\beta} \tau^2_{\gamma,\beta} \quad (3r_T r_V^2) \quad (2317)$$

$$\tau^6_{i,j} = \sum_{\gamma \in A} Y^4_{j,\gamma} \tau^5_{\gamma,i} \quad (2r_T N_o^2) \quad (2305)$$

$$\tau^4_{\gamma,\alpha} = \sum_{\delta \in A} Z_{\gamma,\delta} \tau^3_{\delta,\alpha} \quad (2r_T^2 r_V) \quad (2318)$$

$$\tau_{\gamma,i}^5 = \sum_{\alpha \in B} W_{i,\alpha}^1 \tau_{\gamma,\alpha}^0 \tau_{\gamma,\alpha}^4 \quad (3r_T r_V N_o) \quad (2319)$$

$$\tau_{\gamma,\delta,w}^3 = \sum_{\epsilon \in A} Z_{\epsilon,\gamma} \tau_{\epsilon,\delta,w}^2 \quad (2r_D r_T^3) \quad (2332)$$

$$\tau_{i,j}^6 = \sum_{\gamma \in A} Y_{j,\gamma}^2 \tau_{\gamma,i}^5 \quad (2r_T N_o^2) \quad (2320)$$

$$\tau_{\gamma,\delta,w}^4 = \sum_{i \in O} {}^2D_{i,w}^2 Y_{i,\gamma}^4 Y_{i,\delta}^{2,*} \quad (3r_D r_T^2 N_o) \quad (2333)$$

$$\tau_{\gamma,i}^7 = \sum_{j \in O} Y_{j,\gamma}^4 \tau_{j,i}^6 \quad (2r_T N_o^2) \quad (2321)$$

$$\tau_{\gamma,\alpha}^5 = \sum_{a \in V} W_{a,\alpha}^2 Y_{a,\gamma}^1 \quad (2r_T r_V N_v) \quad (2334)$$

$$\tau_{\gamma,\delta,w}^8 = \sum_{i \in O} {}^2D_{i,w}^2 Y_{i,\delta}^{2,*} \tau_{\gamma,i}^7 \quad (3r_D r_T^2 N_o) \quad (2322)$$

$$\tau_{\gamma,\alpha}^6 = \sum_{i \in O} W_{i,\alpha}^1 Y_{i,\gamma}^2 \quad (2r_T r_V N_o) \quad (2335)$$

$$\tau_{\gamma,\delta,w}^9 = \sum_{a \in V} {}^2D_{a,w}^3 Y_{a,\gamma}^1 Y_{a,\delta}^{3,*} \quad (3r_D r_T^2 N_v) \quad (2323)$$

$$\tau_{\gamma,\alpha}^7 = \sum_{\beta \in B} X_{\beta,\alpha} \tau_{\gamma,\beta}^5 \tau_{\gamma,\beta}^6 \quad (3r_T r_V^2) \quad (2336)$$

$$\tau_{\gamma,\delta,w}^{10} = \sum_{i \in O} {}^2D_{i,w}^4 Y_{i,\gamma}^2 Y_{i,\delta}^{4,*} \quad (3r_D r_T^2 N_o) \quad (2324)$$

$$\tau_{\gamma,\alpha}^8 = \sum_{\delta \in A} Z_{\delta,\gamma} \tau_{\delta,\alpha}^7 \quad (2r_T^2 r_V) \quad (2337)$$

$$\tau_{\gamma,\delta,w}^{11} = \sum_{\epsilon \in A} Z_{\delta,\epsilon}^* \tau_{\gamma,\epsilon,w}^{10} \tau_{\gamma,\epsilon,w}^9 \quad (3r_D r_T^3) \quad (2325)$$

$$\tau_{\gamma,\alpha}^9 = \sum_{i \in O} W_{i,\alpha}^3 Y_{i,\gamma}^4 \quad (2r_T r_V N_o) \quad (2338)$$

$$\tau_{\gamma,\delta,w}^{12} = \sum_{\epsilon \in A} Z_{\epsilon,\gamma} \tau_{\epsilon,\delta,w}^{11} \quad (2r_D r_T^3) \quad (2326)$$

$$\tau_{\gamma,a}^{10} = \sum_{\alpha \in B} W_{a,\alpha}^4 \tau_{\gamma,\alpha}^8 \tau_{\gamma,\alpha}^9 \quad (3r_T r_V N_v) \quad (2339)$$

$${}^{21}R_{a,\gamma} \leftarrow - \sum_{\delta \in A} \sum_{w \in D} \frac{1}{2} {}^2D_{a,w}^1 Y_{a,\delta}^3 \tau_{\delta,\gamma,w}^{12} \tau_{\delta,\gamma,w}^8 \quad (4r_D r_T^2 N_v) \quad (2327)$$

$$\tau_{\gamma,\delta}^{11} = \sum_{a \in V} Y_{a,\delta}^3 \tau_{\gamma,a}^{10} \quad (2r_T^2 N_v) \quad (2340)$$

Raw expression

$$\tau_{\gamma,a}^{12} = \sum_{\delta \in A} Y_{a,\delta}^3 \tau_{\delta,\gamma}^{11} \quad (2r_T^2 N_v) \quad (2341)$$

$${}^{21}R_{a,\epsilon} \leftarrow - \sum_{\gamma \in A} \sum_{i \in O} \sum_{j \in O} \sum_{k \in O} \sum_{l \in O} \sum_{b \in V} \sum_{c \in V} \sum_{d \in V} \frac{1}{2} \quad (2328)$$

$$Y_{i,\epsilon}^{2,*} Z_{\epsilon,\gamma}^* Y_{b,\gamma}^{3,*} Y_{j,\gamma}^{4,*} {}^2D_{a,i,b,j} {}^2T_{b,j,a,k} {}^2T_{c,l,d,i} V_{k,d,l,c}$$

$${}^{21}R_{a,\gamma} \leftarrow - \sum_{\delta \in A} \sum_{w \in D} \frac{1}{2} {}^2D_{a,w}^1 \tau_{\delta,a}^{12} \tau_{\delta,\gamma,w}^3 \tau_{\delta,\gamma,w}^4 \quad (4r_D r_T^2 N_v) \quad (2342)$$

Factorized expression

Raw expression

$$\tau_{\gamma,\delta,w}^0 = \sum_{a \in V} {}^2D_{a,w}^3 Y_{a,\gamma}^1 Y_{a,\delta}^{3,*} \quad (3r_D r_T^2 N_v) \quad (2329)$$

$${}^{21}R_{a,\epsilon} \leftarrow - \sum_{\gamma \in A} \sum_{i \in O} \sum_{j \in O} \sum_{k \in O} \sum_{l \in O} \sum_{b \in V} \sum_{c \in V} \sum_{d \in V} \frac{1}{2} \quad (2343)$$

$$Y_{i,\epsilon}^{2,*} Z_{\epsilon,\gamma}^* Y_{b,\gamma}^{3,*} Y_{j,\gamma}^{4,*} {}^2D_{a,i,b,j} {}^2T_{b,j,d,i} {}^2T_{c,k,a,l} V_{k,c,l,d}$$

$$\tau_{\gamma,\delta,w}^1 = \sum_{i \in O} {}^2D_{i,w}^4 Y_{i,\gamma}^2 Y_{i,\delta}^{4,*} \quad (3r_D r_T^2 N_o) \quad (2330)$$

Factorized expression

$$\tau_{\gamma,\delta,w}^2 = \sum_{\epsilon \in A} Z_{\delta,\epsilon}^* \tau_{\gamma,\epsilon,w}^0 \tau_{\gamma,\epsilon,w}^1 \quad (3r_D r_T^3) \quad (2331)$$

$$\tau_{\gamma,\delta,w}^0 = \sum_{i \in O} {}^2D_{i,w}^2 Y_{i,\gamma}^4 Y_{i,\delta}^{2,*} \quad (3r_D r_T^2 N_o) \quad (2344)$$

$$\tau^1_{\gamma,\delta,w} = \sum_{a \in V} {}^2D^3_{a,w} Y^1_{a,\gamma} Y^{3,*}_{a,\delta} \quad (3r_D r_T^2 N_v) \quad (2345)$$

$$\tau^2_{\gamma,\delta,w} = \sum_{i \in O} {}^2D^4_{i,w} Y^2_{i,\gamma} Y^{4,*}_{i,\delta} \quad (3r_D r_T^2 N_o) \quad (2346)$$

$$\tau^3_{\gamma,\delta,w} = \sum_{\epsilon \in A} Z^*_{\delta,\epsilon} \tau^1_{\gamma,\epsilon,w} \tau^2_{\gamma,\epsilon,w} \quad (3r_D r_T^3) \quad (2347)$$

$$\tau^4_{\gamma,\alpha} = \sum_{a \in V} W^2_{a,\alpha} Y^3_{a,\gamma} \quad (2r_T r_V N_v) \quad (2348)$$

$$\tau^5_{\gamma,\alpha,i} = \sum_{\beta \in B} W^1_{i,\beta} X_{\beta,\alpha} \tau^4_{\gamma,\beta} \quad (3r_T r_V^2 N_o) \quad (2349)$$

$$\tau^6_{\gamma,\alpha} = \sum_{i \in O} W^3_{i,\alpha} Y^4_{i,\gamma} \quad (2r_T r_V N_o) \quad (2350)$$

$$\tau^7_{\gamma,\alpha} = \sum_{a \in V} W^4_{a,\alpha} Y^1_{a,\gamma} \quad (2r_T r_V N_v) \quad (2351)$$

$$\tau^8_{\gamma,\delta,i} = \sum_{\alpha \in B} \tau^6_{\delta,\alpha} \tau^7_{\gamma,\alpha} \tau^5_{\delta,\alpha,i} \quad (3r_T^2 r_V N_o) \quad (2352)$$

$$\tau^9_{\gamma,\delta} = \sum_{i \in O} Y^2_{i,\gamma} \tau^8_{\gamma,\delta,i} \quad (2r_T^2 N_o) \quad (2353)$$

$$\tau^{10}_{\gamma,\delta} = \sum_{\epsilon \in A} Z_{\delta,\epsilon} \tau^9_{\gamma,\epsilon} \quad (2r_T^3) \quad (2354)$$

$$\tau^{11}_{\gamma,\delta} = \sum_{\epsilon \in A} Z_{\epsilon,\delta} \tau^{10}_{\epsilon,\gamma} \quad (2r_T^3) \quad (2355)$$

$$\tau^{12}_{\gamma,\delta,w} = \sum_{\epsilon \in A} \tau^{11}_{\epsilon,\gamma} \tau^3_{\epsilon,\delta,w} \quad (2r_D r_T^3) \quad (2356)$$

$${}^{21}R_{a,\gamma} \leftarrow - \sum_{\delta \in A} \sum_{w \in D} \frac{1}{2} {}^2D^1_{a,w} Y^3_{a,\delta} \tau^0_{\delta,\gamma,w} \tau^{12}_{\delta,\gamma,w} \quad (4r_D r_T^2 N_v) \quad (2357)$$

Raw expression

$${}^{21}R_{a,\epsilon} \leftarrow - \sum_{\gamma \in A} \sum_{i \in O} \sum_{j \in O} \sum_{k \in O} \sum_{l \in O} \sum_{b \in V} \sum_{c \in V} \sum_{d \in V} \frac{1}{2} \quad (2358)$$

$$Y^{2,*}_{i,\epsilon} Z^*_{\epsilon,\gamma} Y^{3,*}_{b,\gamma} Y^{4,*}_{j,\gamma} {}^2D^{a,i,b,j} {}^2T_{b,j,d,l} {}^2T_{c,i,a,k} V_{k,c,l,d}$$

Factorized expression

$$\tau^0_{\gamma,\delta,w} = \sum_{a \in V} {}^2D^3_{a,w} Y^1_{a,\gamma} Y^{3,*}_{a,\delta} \quad (3r_D r_T^2 N_v) \quad (2359)$$

$$\tau^1_{\gamma,\delta,w} = \sum_{i \in O} {}^2D^4_{i,w} Y^2_{i,\gamma} Y^{4,*}_{i,\delta} \quad (3r_D r_T^2 N_o) \quad (2360)$$

$$\tau^2_{\gamma,\delta,w} = \sum_{\epsilon \in A} Z^*_{\delta,\epsilon} \tau^0_{\gamma,\epsilon,w} \tau^1_{\gamma,\epsilon,w} \quad (3r_D r_T^3) \quad (2361)$$

$$\tau^3_{\gamma,\delta,w} = \sum_{\epsilon \in A} Z_{\epsilon,\gamma} \tau^2_{\epsilon,\delta,w} \quad (2r_D r_T^3) \quad (2362)$$

$$\tau^4_{\gamma,\alpha} = \sum_{a \in V} W^4_{a,\alpha} Y^1_{a,\gamma} \quad (2r_T r_V N_v) \quad (2363)$$

$$\tau^5_{\gamma,\alpha} = \sum_{i \in O} W^3_{i,\alpha} Y^2_{i,\gamma} \quad (2r_T r_V N_o) \quad (2364)$$

$$\tau^6_{\gamma,\alpha} = \sum_{\beta \in B} X_{\alpha,\beta} \tau^4_{\gamma,\beta} \tau^5_{\gamma,\beta} \quad (3r_T r_V^2) \quad (2365)$$

$$\tau^7_{\gamma,\alpha} = \sum_{\delta \in A} Z_{\delta,\gamma} \tau^6_{\delta,\alpha} \quad (2r_T^2 r_V) \quad (2366)$$

$$\tau^8_{\gamma,\alpha} = \sum_{a \in V} W^2_{a,\alpha} Y^3_{a,\gamma} \quad (2r_T r_V N_v) \quad (2367)$$

$$\tau^9_{\gamma,i} = \sum_{\alpha \in B} W^1_{i,\alpha} \tau^7_{\gamma,\alpha} \tau^8_{\gamma,\alpha} \quad (3r_T r_V N_o) \quad (2368)$$

$$\tau^{10}_{i,j} = \sum_{\gamma \in A} Y^4_{j,\gamma} \tau^9_{\gamma,i} \quad (2r_T N_o^2) \quad (2369)$$

$$\tau^{11}_{\gamma,i} = \sum_{j \in O} Y^4_{j,\gamma} \tau^{10}_{j,i} \quad (2r_T N_o^2) \quad (2370)$$

$$\tau^{12}_{\gamma,\delta,w} = \sum_{i \in O} {}^2D^2_{i,w} Y^{2,*}_{i,\delta} \tau^{11}_{\gamma,i} \quad (3r_D r_T^2 N_o) \quad (2371)$$

$${}^{21}R_{a,\gamma} \leftarrow - \sum_{\delta \in A} \sum_{w \in D} \frac{1}{2} {}^2D^1_{a,w} Y^3_{a,\delta} \tau^{12}_{\delta,\gamma,w} \tau^3_{\delta,\gamma,w} \quad (4r_D r_T^2 N_v) \quad (2372)$$

Raw expression

$${}^{21}R_{a,\epsilon} \leftarrow - \sum_{\gamma \in A} \sum_{i \in O} \sum_{j \in O} \sum_{k \in O} \sum_{l \in O} \sum_{b \in V} \sum_{c \in V} \sum_{d \in V} \frac{1}{2} \quad (2373)$$

$$Y^{2,*}_{i,\epsilon} Z^*_{\epsilon,\gamma} Y^{3,*}_{b,\gamma} Y^{4,*}_{j,\gamma}$$

$${}^2D^{a,i,b,j} {}^2T_{b,j,d,l} {}^2T_{c,k,a,i} V_{k,d,l,c}$$

Factorized expression

$$\tau^0_{\gamma,\delta,w} = \sum_{i \in O} {}^2D^2_{i,w} Y^4_{i,\gamma} Y^{2,*}_{i,\delta} \quad (3r_D r_T^2 N_o) \quad (2374)$$

$$\tau^1_{\gamma,\alpha} = \sum_{a \in V} W^4_{a,\alpha} Y^1_{a,\gamma} \quad (2r_T r_V N_v) \quad (2375)$$

$$\tau^2_{\gamma,\alpha} = \sum_{i \in O} W^3_{i,\alpha} Y^2_{i,\gamma} \quad (2r_T r_V N_o) \quad (2376)$$

$$\tau^3_{\gamma,\alpha} = \sum_{\beta \in B} X_{\alpha,\beta} \tau^1_{\gamma,\beta} \tau^2_{\gamma,\beta} \quad (3r_T r_V^2) \quad (2377)$$

$$\tau^4_{\gamma,\alpha} = \sum_{\delta \in A} Z_{\delta,\gamma} \tau^3_{\delta,\alpha} \quad (2r_T^2 r_V) \quad (2378)$$

$$\tau^5_{\gamma,\alpha} = \sum_{a \in V} W^2_{a,\alpha} Y^3_{a,\gamma} \quad (2r_T r_V N_v) \quad (2379)$$

$$\tau^6_{\gamma,i} = \sum_{\alpha \in B} W^1_{i,\alpha} \tau^4_{\gamma,\alpha} \tau^5_{\gamma,\alpha} \quad (3r_T r_V N_o) \quad (2380)$$

$$\tau^7_{i,j} = \sum_{\gamma \in A} Y^4_{j,\gamma} \tau^6_{\gamma,i} \quad (2r_T N_o^2) \quad (2381)$$

$$\tau^8_{\gamma,i} = \sum_{j \in O} Y^2_{j,\gamma} \tau^7_{j,i} \quad (2r_T N_o^2) \quad (2382)$$

$$\tau^9_{\gamma,\delta,w} = \sum_{i \in O} {}^2D^4_{i,w} Y^{4,*}_{i,\delta} \tau^8_{\gamma,i} \quad (3r_D r_T^2 N_o) \quad (2383)$$

$$\tau^{10}_{\gamma,\delta,w} = \sum_{a \in V} {}^2D^3_{a,w} Y^1_{a,\gamma} Y^{3,*}_{a,\delta} \quad (3r_D r_T^2 N_v) \quad (2384)$$

$$\tau^{11}_{\gamma,\delta,w} = \sum_{\epsilon \in A} Z^*_{\delta,\epsilon} \tau^{10}_{\gamma,\epsilon,w} \tau^9_{\gamma,\epsilon,w} \quad (3r_D r_T^3) \quad (2385)$$

$$\tau^{12}_{\gamma,\delta,w} = \sum_{\epsilon \in A} Z_{\epsilon,\gamma} \tau^{11}_{\epsilon,\delta,w} \quad (2r_D r_T^3) \quad (2386)$$

$${}^{21}R_{a,\gamma} \leftarrow - \sum_{\delta \in A} \sum_{w \in D} \frac{1}{2} {}^2D^1_{a,w} Y^3_{a,\delta} \tau^0_{\delta,\gamma,w} \tau^{12}_{\delta,\gamma,w} \quad (4r_D r_T^2 N_v) \quad (2387)$$

Raw expression

$${}^{21}R_{a,\epsilon} \leftarrow - \sum_{\gamma \in A} \sum_{i \in O} \sum_{j \in O} \sum_{k \in O} \sum_{l \in O} \sum_{b \in V} \sum_{c \in V} \sum_{d \in V} \frac{1}{2} \quad (2388)$$

$$Y^{2,*}_{i,\epsilon} Z^*_{\epsilon,\gamma} Y^{3,*}_{b,\gamma} Y^{4,*}_{j,\gamma}$$

$${}^2D^{a,i,b,j} {}^2T_{b,k,a,i} {}^2T_{c,j,d,l} V_{k,c,l,d}$$

Factorized expression

$$\tau^0_{\gamma,\delta,w} = \sum_{a \in V} {}^2D^3_{a,w} Y^1_{a,\gamma} Y^{3,*}_{a,\delta} \quad (3r_D r_T^2 N_v) \quad (2389)$$

$$\tau^1_{\gamma,\delta,w} = \sum_{i \in O} {}^2D^4_{i,w} Y^2_{i,\gamma} Y^{4,*}_{i,\delta} \quad (3r_D r_T^2 N_o) \quad (2390)$$

$$\tau^2_{\gamma,\delta,w} = \sum_{\epsilon \in A} Z^*_{\delta,\epsilon} \tau^0_{\gamma,\epsilon,w} \tau^1_{\gamma,\epsilon,w} \quad (3r_D r_T^3) \quad (2391)$$

$$\tau^3_{\gamma,\alpha} = \sum_{a \in V} W^4_{a,\alpha} Y^3_{a,\gamma} \quad (2r_T r_V N_v) \quad (2392)$$

$$\tau^4_{\gamma,\alpha} = \sum_{i \in O} W^3_{i,\alpha} Y^4_{i,\gamma} \quad (2r_T r_V N_o) \quad (2393)$$

$$\tau^5_{\gamma,\alpha} = \sum_{\beta \in B} X_{\alpha,\beta} \tau^3_{\gamma,\beta} \tau^4_{\gamma,\beta} \quad (3r_T r_V^2) \quad (2394)$$

$$\tau^6_{\gamma,\alpha} = \sum_{\delta \in A} Z_{\gamma,\delta} \tau^5_{\delta,\alpha} \quad (2r_T^2 r_V) \quad (2395)$$

$$\tau^7_{\gamma,\alpha} = \sum_{a \in V} W^2_{a,\alpha} Y^1_{a,\gamma} \quad (2r_T r_V N_v) \quad (2396)$$

$$\tau^8_{\gamma,\delta,i} = \sum_{\alpha \in B} W^1_{i,\alpha} \tau^6_{\delta,\alpha} \tau^7_{\gamma,\alpha} \quad (3r_T^2 r_V N_o) \quad (2397)$$

$$\tau^9_{\gamma,\delta,\epsilon} = \sum_{i \in O} Z_{\gamma,\epsilon} Y^4_{i,\epsilon} \tau^8_{\gamma,\delta,i} \quad (3r_T^3 N_o) \quad (2398)$$

$$\tau^{10}_{\gamma,\delta,i} = \sum_{\epsilon \in A} Y^2_{i,\epsilon} \tau^9_{\epsilon,\gamma,\delta} \quad (2r_T^3 N_o) \quad (2399)$$

$$\tau^{11}_{\gamma,\delta,w} = \sum_{\epsilon \in A} \sum_{i \in O} {}^2D^2_{i,w} Y^{2,*}_{i,\delta} \tau^{10}_{\epsilon,\gamma,i} \tau^2_{\epsilon,\delta,w} \quad (4r_D r_T^3 N_o) \quad (2400)$$

$$\tau^{10}_{\gamma,\delta,w} = \sum_{a \in V} {}^2D^3_{a,w} Y^1_{a,\gamma} Y^{3,*}_{a,\delta} \quad (3r_D r_T^2 N_v) \quad (2413)$$

$${}^{21}R_{a,\gamma} \leftarrow - \sum_{\delta \in A} \sum_{w \in D} \frac{1}{2} {}^2D^1_{a,w} Y^3_{a,\delta} \tau^{11}_{\delta,\gamma,w} \quad (3r_D r_T^2 N_v) \quad (2401)$$

$$\tau^{11}_{\gamma,\delta,w} = \sum_{\epsilon \in A} Z^*_{\delta,\epsilon} \tau^{10}_{\gamma,\epsilon,w} \tau^9_{\gamma,\epsilon,w} \quad (3r_D r_T^3) \quad (2414)$$

Raw expression

$$\tau^{12}_{\gamma,\delta,w} = \sum_{\epsilon \in A} Z_{\epsilon,\gamma} \tau^{11}_{\epsilon,\delta,w} \quad (2r_D r_T^3) \quad (2415)$$

$${}^{21}R_{a,\epsilon} \leftarrow - \sum_{\gamma \in A} \sum_{i \in O} \sum_{j \in O} \sum_{k \in O} \sum_{l \in O} \sum_{b \in V} \sum_{c \in V} \sum_{d \in V} \frac{1}{2} \quad (2402)$$

$$\begin{aligned} & Y^{2,*}_{i,\epsilon} Z^*_{\epsilon,\gamma} Y^{3,*}_{b,\gamma} Y^{4,*}_{j,\gamma} \\ & {}^2D^{a,i,b,j}_{b,k,a,i} {}^2T_{b,k,a,i} {}^2T_{c,l,d,j} V_{k,d,l,c} \end{aligned}$$

$${}^{21}R_{a,\gamma} \leftarrow - \sum_{\delta \in A} \sum_{w \in D} \frac{1}{2} {}^2D^1_{a,w} Y^3_{a,\delta} \tau^0_{\delta,\gamma,w} \tau^{12}_{\delta,\gamma,w} \quad (4r_D r_T^2 N_v) \quad (2416)$$

Factorized expression

Raw expression

$$\tau^0_{\gamma,\delta,w} = \sum_{i \in O} {}^2D^2_{i,w} Y^4_{i,\gamma} Y^{2,*}_{i,\delta} \quad (3r_D r_T^2 N_o) \quad (2403)$$

$${}^{21}R_{a,\epsilon} \leftarrow - \sum_{\gamma \in A} \sum_{i \in O} \sum_{j \in O} \sum_{k \in O} \sum_{l \in O} \sum_{b \in V} \sum_{c \in V} \sum_{d \in V} \frac{1}{2} \quad (2417)$$

$$\begin{aligned} & Y^{2,*}_{i,\epsilon} Z^*_{\epsilon,\gamma} Y^{3,*}_{b,\gamma} Y^{4,*}_{j,\gamma} \\ & {}^2D^{a,i,b,j}_{b,k,d,l} {}^2T_{b,k,d,l} {}^2T_{c,j,a,i} V_{k,c,l,d} \end{aligned}$$

$$\tau^1_{\gamma,\alpha} = \sum_{a \in V} W^2_{a,\alpha} Y^1_{a,\gamma} \quad (2r_T r_V N_v) \quad (2404)$$

Factorized expression

$$\tau^2_{\gamma,\alpha} = \sum_{a \in V} W^4_{a,\alpha} Y^3_{a,\gamma} \quad (2r_T r_V N_v) \quad (2405)$$

$$\tau^0_{\gamma,\delta,w} = \sum_{i \in O} {}^2D^2_{i,w} Y^4_{i,\gamma} Y^{2,*}_{i,\delta} \quad (3r_D r_T^2 N_o) \quad (2418)$$

$$\tau^3_{\gamma,\alpha} = \sum_{i \in O} W^3_{i,\alpha} Y^4_{i,\gamma} \quad (2r_T r_V N_o) \quad (2406)$$

$$\tau^1_{\gamma,\delta,w} = \sum_{i \in O} {}^2D^4_{i,w} Y^2_{i,\gamma} Y^{4,*}_{i,\delta} \quad (3r_D r_T^2 N_o) \quad (2419)$$

$$\tau^4_{\gamma,\alpha} = \sum_{\beta \in B} X_{\alpha,\beta} \tau^2_{\gamma,\beta} \tau^3_{\gamma,\beta} \quad (3r_T r_V^2) \quad (2407)$$

$$\tau^2_{\gamma,\alpha} = \sum_{i \in O} W^1_{i,\alpha} Y^2_{i,\gamma} \quad (2r_T r_V N_o) \quad (2420)$$

$$\tau^5_{\gamma,\alpha} = \sum_{\delta \in A} Z_{\gamma,\delta} \tau^4_{\delta,\alpha} \quad (2r_T^2 r_V) \quad (2408)$$

$$\tau^3_{\gamma,\alpha} = \sum_{a \in V} W^4_{a,\alpha} Y^3_{a,\gamma} \quad (2r_T r_V N_v) \quad (2421)$$

$$\tau^6_{\gamma,i} = \sum_{\alpha \in B} W^1_{i,\alpha} \tau^1_{\gamma,\alpha} \tau^5_{\gamma,\alpha} \quad (3r_T r_V N_o) \quad (2409)$$

$$\tau^4_{\gamma,\alpha} = \sum_{i \in O} W^3_{i,\alpha} Y^4_{i,\gamma} \quad (2r_T r_V N_o) \quad (2422)$$

$$\tau^7_{i,j} = \sum_{\gamma \in A} Y^2_{j,\gamma} \tau^6_{\gamma,i} \quad (2r_T N_o^2) \quad (2410)$$

$$\tau^5_{\gamma,\alpha} = \sum_{\beta \in B} X_{\alpha,\beta} \tau^3_{\gamma,\beta} \tau^4_{\gamma,\beta} \quad (3r_T r_V^2) \quad (2423)$$

$$\tau^8_{\gamma,i} = \sum_{j \in O} Y^2_{j,\gamma} \tau^7_{j,i} \quad (2r_T N_o^2) \quad (2411)$$

$$\tau^6_{\gamma,\alpha} = \sum_{\delta \in A} Z_{\gamma,\delta} \tau^5_{\delta,\alpha} \quad (2r_T^2 r_V) \quad (2424)$$

$$\tau^9_{\gamma,\delta,w} = \sum_{i \in O} {}^2D^4_{i,w} Y^{4,*}_{i,\delta} \tau^8_{\gamma,i} \quad (3r_D r_T^2 N_o) \quad (2412)$$

$$\tau^7_{\gamma,a} = \sum_{\alpha \in B} W^2_{a,\alpha} \tau^2_{\gamma,\alpha} \tau^6_{\gamma,\alpha} \quad (3r_T r_V N_v) \quad (2425)$$



$$\tau^8_{a,b} = \sum_{\gamma \in A} Y^1_{b,\gamma} \tau^7_{\gamma,a} \quad (2r_T N_v^2) \quad (2426)$$

$$\tau^9_{\gamma,a} = \sum_{b \in V} Y^1_{b,\gamma} \tau^8_{b,a} \quad (2r_T N_v^2) \quad (2427)$$

$$\tau^{10}_{\gamma,\delta,w} = \sum_{a \in V} {}^2D^3_{a,w} Y^{3,*}_{a,\delta} \tau^9_{\gamma,a} \quad (3r_D r_T^2 N_v) \quad (2428)$$

$$\tau^{11}_{\gamma,\delta,w} = \sum_{\epsilon \in A} Z^*_{\delta,\epsilon} \tau^1_{\gamma,\epsilon,w} \tau^{10}_{\gamma,\epsilon,w} \quad (3r_D r_T^3) \quad (2429)$$

$$\tau^{12}_{\gamma,\delta,w} = \sum_{\epsilon \in A} Z_{\epsilon,\gamma} \tau^{11}_{\epsilon,\delta,w} \quad (2r_D r_T^3) \quad (2430)$$

$${}^{21}R_{a,\gamma} \leftarrow - \sum_{\delta \in A} \sum_{w \in D} \frac{1}{2} {}^2D^1_{a,w} Y^3_{a,\delta} \tau^0_{\delta,\gamma,w} \tau^{12}_{\delta,\gamma,w} \quad (4r_D r_T^2 N_v) \quad (2431)$$

Raw expression

$${}^{21}R_{a,\epsilon} \leftarrow - \sum_{\gamma \in A} \sum_{i \in O} \sum_{j \in O} \sum_{k \in O} \sum_{l \in O} \sum_{b \in V} \sum_{c \in V} \sum_{d \in V} \frac{1}{2} \quad (2432)$$

$$Y^{2,*}_{i,\epsilon} Z^*_{\epsilon,\gamma} Y^{3,*}_{b,\gamma} Y^{4,*}_{j,\gamma} {}^2D^{a,i,b,j} {}^2T_{b,l,d,j} {}^2T_{c,k,a,i} V_{k,c,l,d}$$

Factorized expression

$$\tau^0_{\gamma,\delta,w} = \sum_{i \in O} {}^2D^2_{i,w} Y^4_{i,\gamma} Y^{2,*}_{i,\delta} \quad (3r_D r_T^2 N_o) \quad (2433)$$

$$\tau^1_{\gamma,\delta,w} = \sum_{a \in V} {}^2D^3_{a,w} Y^1_{a,\gamma} Y^{3,*}_{a,\delta} \quad (3r_D r_T^2 N_v) \quad (2434)$$

$$\tau^2_{\gamma,\alpha} = \sum_{a \in V} W^4_{a,\alpha} Y^3_{a,\gamma} \quad (2r_T r_V N_v) \quad (2435)$$

$$\tau^3_{\gamma,\alpha} = \sum_{a \in V} W^2_{a,\alpha} Y^1_{a,\gamma} \quad (2r_T r_V N_v) \quad (2436)$$

$$\tau^4_{\gamma,\alpha} = \sum_{i \in O} W^1_{i,\alpha} Y^2_{i,\gamma} \quad (2r_T r_V N_o) \quad (2437)$$

$$\tau^5_{\gamma,\alpha} = \sum_{\beta \in B} X_{\beta,\alpha} \tau^3_{\gamma,\beta} \tau^4_{\gamma,\beta} \quad (3r_T r_V^2) \quad (2438)$$

$$\tau^6_{\gamma,\alpha} = \sum_{\delta \in A} Z_{\delta,\gamma} \tau^5_{\delta,\alpha} \quad (2r_T^2 r_V) \quad (2439)$$

$$\tau^7_{\gamma,\delta,i} = \sum_{\alpha \in B} W^3_{i,\alpha} \tau^2_{\delta,\alpha} \tau^6_{\gamma,\alpha} \quad (3r_T^2 r_V N_o) \quad (2440)$$

$$\tau^8_{\gamma,\delta,\epsilon} = \sum_{i \in O} Y^2_{i,\gamma} \tau^7_{\delta,\epsilon,i} \quad (2r_T^3 N_o) \quad (2441)$$

$$\tau^9_{\gamma,\delta,i} = \sum_{\epsilon \in A} Z_{\gamma,\epsilon} Y^4_{i,\epsilon} \tau^8_{\gamma,\delta,\epsilon} \quad (3r_T^3 N_o) \quad (2442)$$

$$\tau^{10}_{\gamma,\delta,w} = \sum_{\epsilon \in A} \sum_{i \in O} {}^2D^4_{i,w} Y^{4,*}_{i,\delta} \tau^1_{\epsilon,\delta,w} \tau^9_{\epsilon,\gamma,i} \quad (4r_D r_T^3 N_o) \quad (2443)$$

$$\tau^{11}_{\gamma,\delta,w} = \sum_{\epsilon \in A} Z^*_{\delta,\epsilon} \tau^{10}_{\gamma,\epsilon,w} \quad (2r_D r_T^3) \quad (2444)$$

$${}^{21}R_{a,\gamma} \leftarrow - \sum_{\delta \in A} \sum_{w \in D} \frac{1}{2} {}^2D^1_{a,w} Y^3_{a,\delta} \tau^0_{\delta,\gamma,w} \tau^{11}_{\delta,\gamma,w} \quad (4r_D r_T^2 N_v) \quad (2445)$$

Raw expression

$${}^{21}R_{a,\epsilon} \leftarrow - \sum_{\gamma \in A} \sum_{i \in O} \sum_{j \in O} \sum_{k \in O} \sum_{l \in O} \sum_{b \in V} \sum_{c \in V} \sum_{d \in V} \frac{1}{2} \quad (2446)$$

$$Y^{2,*}_{i,\epsilon} Z^*_{\epsilon,\gamma} Y^{3,*}_{b,\gamma} Y^{4,*}_{j,\gamma} {}^2D^{a,i,b,j} {}^2T_{c,i,a,k} {}^2T_{d,l,b,j} V_{k,c,l,d}$$

Factorized expression

$$\tau^0_{\gamma,\delta,w} = \sum_{a \in V} {}^2D^3_{a,w} Y^3_{a,\gamma} Y^{3,*}_{a,\delta} \quad (3r_D r_T^2 N_v) \quad (2447)$$

$$\tau^1_{\gamma,\delta,w} = \sum_{i \in O} {}^2D^4_{i,w} Y^4_{i,\gamma} Y^{4,*}_{i,\delta} \quad (3r_D r_T^2 N_o) \quad (2448)$$

$$\tau^2_{\gamma,\delta,w} = \sum_{\epsilon \in A} Z^*_{\delta,\epsilon} \tau^0_{\gamma,\epsilon,w} \tau^1_{\gamma,\epsilon,w} \quad (3r_D r_T^3) \quad (2449)$$

$$\tau^3_{\gamma,\alpha} = \sum_{a \in V} W^2_{a,\alpha} Y^1_{a,\gamma} \quad (2r_T r_V N_v) \quad (2450)$$

$$\tau^4_{\gamma,\alpha} = \sum_{a \in V} W^4_{a,\alpha} Y^1_{a,\gamma} \quad (2r_T r_V N_v) \quad (2451)$$

$$\tau^5_{\gamma,\alpha} = \sum_{i \in O} W^3_{i,\alpha} Y^2_{i,\gamma} \quad (2r_T r_V N_o) \quad (2452)$$

$$\tau^4_{\gamma,\delta,w} = \sum_{\epsilon \in A} Z_{\gamma,\epsilon} \tau^3_{\epsilon,\delta,w} \quad (2r_D r_T^3) \quad (2465)$$

$$\tau^6_{\gamma,\alpha} = \sum_{\beta \in B} X_{\alpha,\beta} \tau^4_{\gamma,\beta} \tau^5_{\gamma,\beta} \quad (3r_T r_V^2) \quad (2453)$$

$$\tau^5_{\gamma,\alpha} = \sum_{a \in V} W^2_{a,\alpha} Y^1_{a,\gamma} \quad (2r_T r_V N_v) \quad (2466)$$

$$\tau^7_{\gamma,\alpha} = \sum_{\delta \in A} Z_{\delta,\gamma} \tau^6_{\delta,\alpha} \quad (2r_T^2 r_V) \quad (2454)$$

$$\tau^6_{\gamma,\alpha} = \sum_{i \in O} W^1_{i,\alpha} Y^2_{i,\gamma} \quad (2r_T r_V N_o) \quad (2467)$$

$$\tau^8_{\gamma,\delta,i} = \sum_{\alpha \in B} W^1_{i,\alpha} \tau^3_{\gamma,\alpha} \tau^7_{\delta,\alpha} \quad (3r_T^2 r_V N_o) \quad (2455)$$

$$\tau^7_{\gamma,\alpha} = \sum_{\beta \in B} X_{\beta,\alpha} \tau^5_{\gamma,\beta} \tau^6_{\gamma,\beta} \quad (3r_T r_V^2) \quad (2468)$$

$$\tau^9_{\gamma,\delta,\epsilon} = \sum_{i \in O} Z_{\gamma,\delta} Y^4_{i,\delta} \tau^8_{\gamma,\epsilon,i} \quad (3r_T^3 N_o) \quad (2456)$$

$$\tau^8_{\gamma,\alpha} = \sum_{\delta \in A} Z_{\delta,\gamma} \tau^7_{\delta,\alpha} \quad (2r_T^2 r_V) \quad (2469)$$

$$\tau^{10}_{\gamma,\delta,i} = \sum_{\epsilon \in A} Y^2_{i,\epsilon} \tau^9_{\epsilon,\gamma,\delta} \quad (2r_T^3 N_o) \quad (2457)$$

$$\tau^9_{\gamma,\alpha} = \sum_{i \in O} W^3_{i,\alpha} Y^4_{i,\gamma} \quad (2r_T r_V N_o) \quad (2470)$$

$$\tau^{11}_{\gamma,\delta,w} = \sum_{\epsilon \in A} \sum_{i \in O} {}^2D^2_{i,w} Y^{2,*}_{i,\delta} \tau^{10}_{\gamma,\epsilon,i} \tau^2_{\epsilon,\delta,w} \quad (4r_D r_T^3 N_o) \quad (2458)$$

$$\tau^{10}_{\gamma,a} = \sum_{\alpha \in B} W^4_{a,\alpha} \tau^8_{\gamma,\alpha} \tau^9_{\gamma,\alpha} \quad (3r_T r_V N_v) \quad (2471)$$

$${}^{21}R_{a,\gamma} \leftarrow - \sum_{\delta \in A} \sum_{w \in D} \frac{1}{2} {}^2D^1_{a,w} Y^3_{a,\delta} \tau^{11}_{\delta,\gamma,w} \quad (3r_D r_T^2 N_v) \quad (2459)$$

$$\tau^{11}_{\gamma,\delta} = \sum_{a \in V} Y^1_{a,\gamma} \tau^{10}_{\delta,a} \quad (2r_T^2 N_v) \quad (2472)$$

Raw expression

$$\tau^{12}_{\gamma,a} = \sum_{\delta \in A} Y^3_{a,\delta} \tau^{11}_{\gamma,\delta} \quad (2r_T^2 N_v) \quad (2473)$$

$${}^{21}R_{a,\epsilon} \leftarrow - \sum_{\gamma \in A} \sum_{i \in O} \sum_{j \in O} \sum_{k \in O} \sum_{l \in O} \sum_{b \in V} \sum_{c \in V} \sum_{d \in V} \frac{1}{2} \quad (2460)$$

$$Y^{2,*}_{i,\epsilon} Z^*_{\epsilon,\gamma} Y^{3,*}_{b,\gamma} Y^{4,*}_{j,\gamma} {}^2D^{a,i,b,j} {}^2T_{c,j,a,i} {}^2T_{d,k,b,l} V_{k,d,l,c}$$

$${}^{21}R_{a,\gamma} \leftarrow - \sum_{\delta \in A} \sum_{w \in D} \frac{1}{2} {}^2D^1_{a,w} \tau^{12}_{\delta,a} \tau^0_{\delta,\gamma,w} \tau^4_{\delta,\gamma,w} \quad (4r_D r_T^2 N_v) \quad (2474)$$

Factorized expression

Raw expression

$$\tau^0_{\gamma,\delta,w} = \sum_{i \in O} {}^2D^2_{i,w} Y^2_{i,\gamma} Y^{2,*}_{i,\delta} \quad (3r_D r_T^2 N_o) \quad (2461)$$

$${}^{21}R_{a,\epsilon} \leftarrow - \sum_{\gamma \in A} \sum_{i \in O} \sum_{j \in O} \sum_{k \in O} \sum_{l \in O} \sum_{b \in V} \sum_{c \in V} \sum_{d \in V} \frac{1}{2} \quad (2475)$$

$$Y^{2,*}_{i,\epsilon} Z^*_{\epsilon,\gamma} Y^{3,*}_{b,\gamma} Y^{4,*}_{j,\gamma} {}^2D^{a,i,b,j} {}^2T_{c,k,a,i} {}^2T_{d,j,b,l} V_{k,c,l,d}$$

$$\tau^1_{\gamma,\delta,w} = \sum_{a \in V} {}^2D^3_{a,w} Y^3_{a,\gamma} Y^{3,*}_{a,\delta} \quad (3r_D r_T^2 N_v) \quad (2462)$$

Factorized expression

$$\tau^2_{\gamma,\delta,w} = \sum_{i \in O} {}^2D^4_{i,w} Y^4_{i,\gamma} Y^{4,*}_{i,\delta} \quad (3r_D r_T^2 N_o) \quad (2463)$$

$$\tau^0_{\gamma,\delta,w} = \sum_{i \in O} {}^2D^2_{i,w} Y^4_{i,\gamma} Y^{2,*}_{i,\delta} \quad (3r_D r_T^2 N_o) \quad (2476)$$

$$\tau^3_{\gamma,\delta,w} = \sum_{\epsilon \in A} Z^*_{\delta,\epsilon} \tau^1_{\gamma,\epsilon,w} \tau^2_{\gamma,\epsilon,w} \quad (3r_D r_T^3) \quad (2464)$$

$$\tau^1_{\gamma,\delta,w} = \sum_{a \in V} {}^2D^3_{a,w} Y^3_{a,\gamma} Y^{3,*}_{a,\delta} \quad (3r_D r_T^2 N_v) \quad (2477)$$

$$\tau^2_{\gamma,\alpha} = \sum_{a \in V} W^2_{a,\alpha} Y^1_{a,\gamma} \quad (2r_T r_V N_v) \quad (2478)$$

$$\tau^3_{\gamma,\alpha} = \sum_{i \in O} W^1_{i,\alpha} Y^2_{i,\gamma} \quad (2r_T r_V N_o) \quad (2479)$$

$$\tau^4_{\gamma,\alpha} = \sum_{\beta \in B} X_{\beta,\alpha} \tau^2_{\gamma,\beta} \tau^3_{\gamma,\beta} \quad (3r_T r_V^2) \quad (2480)$$

$$\tau^5_{\gamma,\alpha} = \sum_{\delta \in A} Z_{\delta,\gamma} \tau^4_{\delta,\alpha} \quad (2r_T^2 r_V) \quad (2481)$$

$$\tau^6_{\gamma,\alpha} = \sum_{a \in V} W^4_{a,\alpha} Y^1_{a,\gamma} \quad (2r_T r_V N_v) \quad (2482)$$

$$\tau^7_{\gamma,\delta,i} = \sum_{\alpha \in B} W^3_{i,\alpha} \tau^5_{\delta,\alpha} \tau^6_{\gamma,\alpha} \quad (3r_T^2 r_V N_o) \quad (2483)$$

$$\tau^8_{\gamma,\delta,\epsilon} = \sum_{i \in O} Z_{\gamma,\delta} Y^4_{i,\delta} \tau^7_{\gamma,\epsilon,i} \quad (3r_T^3 N_o) \quad (2484)$$

$$\tau^9_{\gamma,\delta,i} = \sum_{\epsilon \in A} Y^2_{i,\epsilon} \tau^8_{\epsilon,\gamma,\delta} \quad (2r_T^3 N_o) \quad (2485)$$

$$\tau^{10}_{\gamma,\delta,w} = \sum_{\epsilon \in A} \sum_{i \in O} {}^2D^4_{i,w} Y^{4,*}_{i,\delta} \tau^1_{\epsilon,\delta,w} \tau^9_{\epsilon,\gamma,i} \quad (4r_D r_T^3 N_o) \quad (2486)$$

$$\tau^{11}_{\gamma,\delta,w} = \sum_{\epsilon \in A} Z^*_{\delta,\epsilon} \tau^{10}_{\gamma,\epsilon,w} \quad (2r_D r_T^3) \quad (2487)$$

$${}^{21}R_{a,\gamma} \leftarrow - \sum_{\delta \in A} \sum_{w \in D} \frac{1}{2} {}^2D^1_{a,w} Y^3_{a,\delta} \tau^0_{\delta,\gamma,w} \tau^{11}_{\delta,\gamma,w} \quad (4r_D r_T^2 N_v) \quad (2488)$$

Raw expression

$${}^{21}R_{a,\epsilon} \leftarrow - \sum_{\gamma \in A} \sum_{i \in O} \sum_{j \in O} \sum_{k \in O} \sum_{l \in O} \sum_{b \in V} \sum_{c \in V} \sum_{d \in V} \frac{1}{2} Y^{2,*}_{i,\epsilon} Z^*_{\epsilon,\gamma} Y^{3,*}_{b,\gamma} Y^{4,*}_{j,\gamma} {}^2D^{a,i,b,j} {}^2T_{c,k,a,i} {}^2T_{d,l,b,j} V_{k,d,l,c} \quad (2489)$$

Factorized expression

$$\tau^0_{\gamma,\delta,w} = \sum_{i \in O} {}^2D^2_{i,w} Y^4_{i,\gamma} Y^{2,*}_{i,\delta} \quad (3r_D r_T^2 N_o) \quad (2490)$$

$$\tau^1_{\gamma,\delta,w} = \sum_{i \in O} {}^2D^4_{i,w} Y^2_{i,\gamma} Y^{4,*}_{i,\delta} \quad (3r_D r_T^2 N_o) \quad (2491)$$

$$\tau^2_{\gamma,\alpha} = \sum_{a \in V} W^2_{a,\alpha} Y^1_{a,\gamma} \quad (2r_T r_V N_v) \quad (2492)$$

$$\tau^3_{\gamma,\alpha} = \sum_{i \in O} W^1_{i,\alpha} Y^2_{i,\gamma} \quad (2r_T r_V N_o) \quad (2493)$$

$$\tau^4_{\gamma,\alpha} = \sum_{\beta \in B} X_{\beta,\alpha} \tau^2_{\gamma,\beta} \tau^3_{\gamma,\beta} \quad (3r_T r_V^2) \quad (2494)$$

$$\tau^5_{\gamma,\alpha} = \sum_{\delta \in A} Z_{\delta,\gamma} \tau^4_{\delta,\alpha} \quad (2r_T^2 r_V) \quad (2495)$$

$$\tau^6_{\gamma,\alpha} = \sum_{i \in O} W^3_{i,\alpha} Y^4_{i,\gamma} \quad (2r_T r_V N_o) \quad (2496)$$

$$\tau^7_{\gamma,a} = \sum_{\alpha \in B} W^4_{a,\alpha} \tau^5_{\gamma,\alpha} \tau^6_{\gamma,\alpha} \quad (3r_T r_V N_v) \quad (2497)$$

$$\tau^8_{\gamma,\delta} = \sum_{a \in V} Y^1_{a,\gamma} \tau^7_{\delta,a} \quad (2r_T^2 N_v) \quad (2498)$$

$$\tau^9_{\gamma,a} = \sum_{\delta \in A} Y^3_{a,\delta} \tau^8_{\gamma,\delta} \quad (2r_T^2 N_v) \quad (2499)$$

$$\tau^{10}_{\gamma,\delta,w} = \sum_{a \in V} {}^2D^3_{a,w} Y^{3,*}_{a,\delta} \tau^9_{\gamma,a} \quad (3r_D r_T^2 N_v) \quad (2500)$$

$$\tau^{11}_{\gamma,\delta,w} = \sum_{\epsilon \in A} Z^*_{\delta,\epsilon} \tau^1_{\gamma,\epsilon,w} \tau^{10}_{\gamma,\epsilon,w} \quad (3r_D r_T^3) \quad (2501)$$

$$\tau^{12}_{\gamma,\delta,w} = \sum_{\epsilon \in A} Z_{\epsilon,\gamma} \tau^{11}_{\epsilon,\delta,w} \quad (2r_D r_T^3) \quad (2502)$$

$${}^{21}R_{a,\gamma} \leftarrow - \sum_{\delta \in A} \sum_{w \in D} \frac{1}{2} {}^2D^1_{a,w} Y^3_{a,\delta} \tau^0_{\delta,\gamma,w} \tau^{12}_{\delta,\gamma,w} \quad (4r_D r_T^2 N_v) \quad (2503)$$

Raw expression

$${}^{21}R_{a,\epsilon} \leftarrow - \sum_{\gamma \in A} \sum_{i \in O} \sum_{j \in O} \sum_{k \in O} \sum_{l \in O} \sum_{b \in V} \sum_{c \in V} \sum_{d \in V} \frac{1}{2} Y^{2,*}_{i,\epsilon} Z^*_{\epsilon,\gamma} Y^{3,*}_{b,\gamma} Y^{4,*}_{j,\gamma} {}^2D^{a,i,b,j} {}^2T_{c,k,a,l} {}^2T_{d,i,b,j} V_{k,c,l,d} \quad (2504)$$

Factorized expression

$$\tau^0_{\gamma,\delta,w} = \sum_{i \in O} {}^2D^2_{i,w} Y^4_{i,\gamma} Y^{2,*}_{i,\delta} \quad (3r_D r_T^2 N_o) \quad (2505)$$

$$\tau^1_{\gamma,\delta,w} = \sum_{a \in V} {}^2D^3_{a,w} Y^3_{a,\gamma} Y^{3,*}_{a,\delta} \quad (3r_D r_T^2 N_v) \quad (2506)$$

$$\tau^2_{\gamma,\delta,w} = \sum_{i \in O} {}^2D^4_{i,w} Y^4_{i,\gamma} Y^{4,*}_{i,\delta} \quad (3r_D r_T^2 N_o) \quad (2507)$$

$$\tau^3_{\gamma,\delta,w} = \sum_{\epsilon \in A} Z^*_{\delta,\epsilon} \tau^1_{\gamma,\epsilon,w} \tau^2_{\gamma,\epsilon,w} \quad (3r_D r_T^3) \quad (2508)$$

$$\tau^4_{\gamma,\alpha} = \sum_{a \in V} W^2_{a,\alpha} Y^1_{a,\gamma} \quad (2r_T r_V N_v) \quad (2509)$$

$$\tau^5_{\gamma,\alpha,i} = \sum_{\beta \in B} W^1_{i,\beta} X_{\beta,\alpha} \tau^4_{\gamma,\beta} \quad (3r_T r_V^2 N_o) \quad (2510)$$

$$\tau^6_{\gamma,\alpha} = \sum_{i \in O} W^3_{i,\alpha} Y^2_{i,\gamma} \quad (2r_T r_V N_o) \quad (2511)$$

$$\tau^7_{\gamma,\alpha} = \sum_{a \in V} W^4_{a,\alpha} Y^1_{a,\gamma} \quad (2r_T r_V N_v) \quad (2512)$$

$$\tau^8_{\gamma,\delta,i} = \sum_{\alpha \in B} \tau^6_{\gamma,\alpha} \tau^7_{\delta,\alpha} \tau^5_{\gamma,\alpha,i} \quad (3r_T^2 r_V N_o) \quad (2513)$$

$$\tau^9_{\gamma,\delta} = \sum_{i \in O} Y^2_{i,\delta} \tau^8_{\gamma,\delta,i} \quad (2r_T^2 N_o) \quad (2514)$$

$$\tau^{10}_{\gamma,\delta} = \sum_{\epsilon \in A} Z_{\epsilon,\delta} \tau^9_{\gamma,\epsilon} \quad (2r_T^3) \quad (2515)$$

$$\tau^{11}_{\gamma,\delta} = \sum_{\epsilon \in A} Z_{\epsilon,\gamma} \tau^{10}_{\epsilon,\delta} \quad (2r_T^3) \quad (2516)$$

$$\tau^{12}_{\gamma,\delta,w} = \sum_{\epsilon \in A} \tau^{11}_{\epsilon,\gamma} \tau^3_{\epsilon,\delta,w} \quad (2r_D r_T^3) \quad (2517)$$

$${}^{21}R_{a,\gamma} \leftarrow - \sum_{\delta \in A} \sum_{w \in D} \frac{1}{2} {}^2D^1_{a,w} Y^3_{a,\delta} \tau^0_{\delta,\gamma,w} \tau^{12}_{\delta,\gamma,w} \quad (4r_D r_T^2 N_v) \quad (2518)$$

Raw expression

$${}^{21}R_{a,\epsilon} \leftarrow \sum_{\gamma \in A} \sum_{i \in O} \sum_{j \in O} \sum_{k \in O} \sum_{l \in O} \sum_{b \in V} \sum_{c \in V} \sum_{d \in V} \frac{1}{4} Y^{2,*}_{i,\epsilon} Z^*_{\epsilon,\gamma} Y^{3,*}_{b,\gamma} Y^{4,*}_{j,\gamma} {}^2D^{a,i,b,j}_{a,i,b,k} {}^2T_{a,i,b,k} {}^2T_{c,j,d,l} V_{k,d,l,c} \quad (2519)$$

Factorized expression

$$\tau^0_{\gamma,\delta,w} = \sum_{i \in O} {}^2D^2_{i,w} Y^2_{i,\gamma} Y^{2,*}_{i,\delta} \quad (3r_D r_T^2 N_o) \quad (2520)$$

$$\tau^1_{\gamma,\alpha} = \sum_{a \in V} W^2_{a,\alpha} Y^3_{a,\gamma} \quad (2r_T r_V N_v) \quad (2521)$$

$$\tau^2_{\gamma,\alpha,i} = \sum_{\beta \in B} W^1_{i,\beta} X_{\beta,\alpha} \tau^1_{\gamma,\beta} \quad (3r_T r_V^2 N_o) \quad (2522)$$

$$\tau^3_{\gamma,\alpha} = \sum_{i \in O} W^3_{i,\alpha} Y^4_{i,\gamma} \quad (2r_T r_V N_o) \quad (2523)$$

$$\tau^4_{\gamma,\alpha} = \sum_{\delta \in A} \sum_{i \in O} Y^2_{i,\gamma} Z_{\gamma,\delta} \tau^3_{\delta,\alpha} \tau^2_{\delta,\alpha,i} \quad (4r_T^2 r_V N_o) \quad (2524)$$

$$\tau^5_{\gamma,a} = \sum_{\alpha \in B} W^4_{a,\alpha} \tau^4_{\gamma,\alpha} \quad (2r_T r_V N_v) \quad (2525)$$

$$\tau^6_{\gamma,\delta} = \sum_{a \in V} Y^3_{a,\delta} \tau^5_{\gamma,a} \quad (2r_T^2 N_v) \quad (2526)$$

$$\tau^7_{\gamma,a} = \sum_{\delta \in A} Y^1_{a,\delta} \tau^6_{\delta,\gamma} \quad (2r_T^2 N_v) \quad (2527)$$

$$\tau^8_{\gamma,\delta,w} = \sum_{a \in V} {}^2D^3_{a,w} Y^{3,*}_{a,\delta} \tau^7_{\gamma,a} \quad (3r_D r_T^2 N_v) \quad (2528)$$

$$\tau^9_{\gamma,\delta,w} = \sum_{i \in O} {}^2D^4_{i,w} Y^4_{i,\gamma} Y^{4,*}_{i,\delta} \quad (3r_D r_T^2 N_o) \quad (2529)$$

$$\tau^{10}_{\gamma,\delta,w} = \sum_{\epsilon \in A} Z^*_{\delta,\epsilon} \tau^8_{\gamma,\epsilon,w} \tau^9_{\gamma,\epsilon,w} \quad (3r_D r_T^3) \quad (2530)$$

$$\tau^{11}_{\gamma,\delta,w} = \sum_{\epsilon \in A} Z_{\gamma,\epsilon} \tau^{10}_{\epsilon,\delta,w} \quad (2r_D r_T^3) \quad (2531)$$

$${}^{21}R_{a,\gamma} \leftarrow \sum_{\delta \in A} \sum_{w \in D} \frac{1}{4} {}^2D^1_{a,w} Y^1_{a,\delta} \tau^0_{\delta,\gamma,w} \tau^{11}_{\delta,\gamma,w} \quad (4r_D r_T^2 N_v) \quad (2532)$$

Raw expression

$${}^{21}R_{a,\epsilon} \leftarrow \sum_{\gamma \in A} \sum_{i \in O} \sum_{j \in O} \sum_{k \in O} \sum_{l \in O} \sum_{b \in V} \sum_{c \in V} \sum_{d \in V} \frac{1}{4} Y^{2,*}_{i,\epsilon} Z^*_{\epsilon,\gamma} Y^{3,*}_{b,\gamma} Y^{4,*}_{j,\gamma} {}^2D^{a,i,b,j} {}^2T_{a,i,b,k} {}^2T_{c,l,d,j} V_{k,c,l,d} \quad (2533)$$

Factorized expression

$$\tau^0_{\gamma,\delta,w} = \sum_{i \in O} {}^2D^2_{i,w} Y^2_{i,\gamma} Y^{2,*}_{i,\delta} \quad (3r_D r_T^2 N_o) \quad (2534)$$

$$\tau^1_{\gamma,\delta,w} = \sum_{a \in V} {}^2D^3_{a,w} Y^1_{a,\gamma} Y^{3,*}_{a,\delta} \quad (3r_D r_T^2 N_v) \quad (2535)$$

$$\tau^2_{\gamma,\alpha} = \sum_{a \in V} W^4_{a,\alpha} Y^3_{a,\gamma} \quad (2r_T r_V N_v) \quad (2536)$$

$$\tau^3_{\gamma,\alpha,i} = \sum_{\beta \in B} X_{\alpha,\beta} W^3_{i,\beta} \tau^2_{\gamma,\beta} \quad (3r_T r_V^2 N_o) \quad (2537)$$

$$\tau^4_{\gamma,\alpha} = \sum_{i \in O} W^1_{i,\alpha} Y^4_{i,\gamma} \quad (2r_T r_V N_o) \quad (2538)$$

$$\tau^5_{\gamma,\alpha} = \sum_{a \in V} W^2_{a,\alpha} Y^3_{a,\gamma} \quad (2r_T r_V N_v) \quad (2539)$$

$$\tau^6_{\gamma,\delta,i} = \sum_{\alpha \in B} \tau^4_{\gamma,\alpha} \tau^5_{\delta,\alpha} \tau^3_{\gamma,\alpha,i} \quad (3r_T^2 r_V N_o) \quad (2540)$$

$$\tau^7_{\gamma,\delta,\epsilon} = \sum_{i \in O} Y^2_{i,\gamma} Z_{\gamma,\delta} \tau^6_{\epsilon,\delta,i} \quad (3r_T^3 N_o) \quad (2541)$$

$$\tau^8_{\gamma,\delta,i} = \sum_{\epsilon \in A} Y^4_{i,\epsilon} \tau^7_{\gamma,\epsilon,\delta} \quad (2r_T^3 N_o) \quad (2542)$$

$$\tau^9_{\gamma,\delta,w} = \sum_{\epsilon \in A} \sum_{i \in O} {}^2D^4_{i,w} Y^{4,*}_{i,\delta} \tau^1_{\epsilon,\delta,w} \tau^8_{\epsilon,\gamma,i} \quad (4r_D r_T^3 N_o) \quad (2543)$$

$$\tau^{10}_{\gamma,\delta,w} = \sum_{\epsilon \in A} Z^*_{\delta,\epsilon} \tau^9_{\gamma,\epsilon,w} \quad (2r_D r_T^3) \quad (2544)$$

$$\tau^{11}_{\gamma,\delta,w} = \sum_{\epsilon \in A} Z_{\gamma,\epsilon} \tau^{10}_{\epsilon,\delta,w} \quad (2r_D r_T^3) \quad (2545)$$

$${}^{21}R_{a,\gamma} \leftarrow \sum_{\delta \in A} \sum_{w \in D} \frac{1}{4} {}^2D^1_{a,w} Y^1_{a,\delta} \tau^0_{\delta,\gamma,w} \tau^{11}_{\delta,\gamma,w} \quad (4r_D r_T^2 N_v) \quad (2546)$$

Raw expression

$${}^{21}R_{a,\epsilon} \leftarrow \sum_{\gamma \in A} \sum_{i \in O} \sum_{j \in O} \sum_{k \in O} \sum_{l \in O} \sum_{b \in V} \sum_{c \in V} \sum_{d \in V} \frac{1}{4} Y^{2,*}_{i,\epsilon} Z^*_{\epsilon,\gamma} Y^{3,*}_{b,\gamma} Y^{4,*}_{j,\gamma} {}^2D^{a,i,b,j} {}^2T_{a,i,c,j} {}^2T_{b,k,d,l} V_{k,d,l,c} \quad (2547)$$

Factorized expression

$$\tau^0_{\gamma,\delta,w} = \sum_{a \in V} {}^2D^3_{a,w} Y^1_{a,\gamma} Y^{3,*}_{a,\delta} \quad (3r_D r_T^2 N_v) \quad (2548)$$

$$\tau^1_{\gamma,\delta,w} = \sum_{i \in O} {}^2D^4_{i,w} Y^2_{i,\gamma} Y^{4,*}_{i,\delta} \quad (3r_D r_T^2 N_o) \quad (2549)$$

$$\tau^2_{\gamma,\delta,w} = \sum_{\epsilon \in A} Z^*_{\delta,\epsilon} \tau^0_{\gamma,\epsilon,w} \tau^1_{\gamma,\epsilon,w} \quad (3r_D r_T^3) \quad (2550)$$

$$\tau^3_{\gamma,\delta,w} = \sum_{\epsilon \in A} Z_{\epsilon,\gamma} \tau^2_{\epsilon,\delta,w} \quad (2r_D r_T^3) \quad (2551)$$

$$\tau^4_{\gamma,\alpha} = \sum_{a \in V} W^2_{a,\alpha} Y^3_{a,\gamma} \quad (2r_T r_V N_v) \quad (2552)$$

$$\tau^5_{\gamma,\alpha,i} = \sum_{\beta \in B} W^1_{i,\beta} X_{\beta,\alpha} \tau^4_{\gamma,\beta} \quad (3r_T r_V^2 N_o) \quad (2553)$$

$$\tau^6_{\gamma,\alpha} = \sum_{i \in O} W^3_{i,\alpha} Y^4_{i,\gamma} \quad (2r_T r_V N_o) \quad (2554)$$

$$\tau^7_{\gamma,\alpha} = \sum_{a \in V} W^4_{a,\alpha} Y^3_{a,\gamma} \quad (2r_T r_V N_v) \quad (2555)$$

$$\tau^8_{\gamma,\delta,i} = \sum_{\alpha \in B} \tau^6_{\gamma,\alpha} \tau^7_{\delta,\alpha} \tau^5_{\gamma,\alpha,i} \quad (3r_T^2 r_V N_o) \quad (2556)$$

$$\tau^9_{\gamma,\delta,\epsilon} = \sum_{i \in O} Y^2_{i,\gamma} Z_{\gamma,\delta} \tau^8_{\epsilon,\delta,i} \quad (3r_T^3 N_o) \quad (2557)$$

$$\tau^{10}_{\gamma,\delta,i} = \sum_{\epsilon \in A} Y^4_{i,\epsilon} \tau^9_{\gamma,\epsilon,\delta} \quad (2r_T^3 N_o) \quad (2558)$$

$$\tau^{11}_{\gamma,\delta,w} = \sum_{\epsilon \in A} \sum_{i \in O} {}^2D^2_{i,w} Y^{2,*}_{i,\delta} \tau^{10}_{\gamma,\epsilon,i} \tau^3_{\epsilon,\delta,w} \quad (4r_D r_T^3 N_o) \quad (2559)$$

$$\tau^{10}_{\gamma,\delta} = \sum_{a \in V} Y^3_{a,\delta} \tau^9_{\gamma,a} \quad (2r_T^2 N_v) \quad (2572)$$

$${}^{21}R_{a,\gamma} \leftarrow \sum_{\delta \in A} \sum_{w \in D} \frac{1}{4} {}^2D^1_{a,w} Y^1_{a,\delta} \tau^{11}_{\delta,\gamma,w} \quad (3r_D r_T^2 N_v) \quad (2560)$$

$$\tau^{11}_{\gamma,a} = \sum_{\delta \in A} Y^1_{a,\delta} \tau^{10}_{\delta,\gamma} \quad (2r_T^2 N_v) \quad (2573)$$

$${}^{21}R_{a,\gamma} \leftarrow \sum_{\delta \in A} \sum_{w \in D} \frac{1}{4} {}^2D^1_{a,w} \tau^{11}_{\delta,a} \tau^3_{\delta,\gamma,w} \tau^4_{\delta,\gamma,w} \quad (4r_D r_T^2 N_v) \quad (2574)$$

Raw expression

$${}^{21}R_{a,\epsilon} \leftarrow \sum_{\gamma \in A} \sum_{i \in O} \sum_{j \in O} \sum_{k \in O} \sum_{l \in O} \sum_{b \in V} \sum_{c \in V} \sum_{d \in V} \frac{1}{4} Y^{2,*}_{i,\epsilon} Z^*_{\epsilon,\gamma} Y^{3,*}_{b,\gamma} Y^{4,*}_{j,\gamma} {}^2D^{a,i,b,j} {}^2T_{a,i,c,j} {}^2T_{d,k,b,l} V_{k,c,l,d} \quad (2561)$$

Raw expression

$${}^{21}R_{a,\epsilon} \leftarrow \sum_{\gamma \in A} \sum_{i \in O} \sum_{j \in O} \sum_{k \in O} \sum_{l \in O} \sum_{b \in V} \sum_{c \in V} \sum_{d \in V} \frac{1}{4} Y^{2,*}_{i,\epsilon} Z^*_{\epsilon,\gamma} Y^{3,*}_{b,\gamma} Y^{4,*}_{j,\gamma} {}^2D^{a,i,b,j} {}^2T_{a,i,c,k} {}^2T_{b,l,d,j} V_{k,d,l,c} \quad (2575)$$

Factorized expression

$$\tau^0_{\gamma,\delta,w} = \sum_{a \in V} {}^2D^3_{a,w} Y^1_{a,\gamma} Y^{3,*}_{a,\delta} \quad (3r_D r_T^2 N_v) \quad (2562)$$

Factorized expression

$$\tau^0_{\gamma,\alpha} = \sum_{a \in V} W^2_{a,\alpha} Y^3_{a,\gamma} \quad (2r_T r_V N_v) \quad (2576)$$

$$\tau^1_{\gamma,\delta,w} = \sum_{i \in O} {}^2D^4_{i,w} Y^2_{i,\gamma} Y^{4,*}_{i,\delta} \quad (3r_D r_T^2 N_o) \quad (2563)$$

$$\tau^1_{\gamma,\alpha,i} = \sum_{\beta \in B} W^1_{i,\beta} X_{\beta,\alpha} \tau^0_{\gamma,\beta} \quad (3r_T r_V^2 N_o) \quad (2577)$$

$$\tau^2_{\gamma,\delta,w} = \sum_{\epsilon \in A} Z^*_{\delta,\epsilon} \tau^0_{\gamma,\epsilon,w} \tau^1_{\gamma,\epsilon,w} \quad (3r_D r_T^3) \quad (2564)$$

$$\tau^2_{\gamma,\delta,\alpha} = \sum_{i \in O} Y^2_{i,\gamma} \tau^1_{\delta,\alpha,i} \quad (2r_T^2 r_V N_o) \quad (2578)$$

$$\tau^3_{\gamma,\delta,w} = \sum_{\epsilon \in A} Z_{\epsilon,\gamma} \tau^2_{\epsilon,\delta,w} \quad (2r_D r_T^3) \quad (2565)$$

$$\tau^3_{\gamma,\delta,w} = \sum_{a \in V} {}^2D^3_{a,w} Y^1_{a,\gamma} Y^{3,*}_{a,\delta} \quad (3r_D r_T^2 N_v) \quad (2579)$$

$$\tau^4_{\gamma,\delta,w} = \sum_{i \in O} {}^2D^2_{i,w} Y^4_{i,\gamma} Y^{2,*}_{i,\delta} \quad (3r_D r_T^2 N_o) \quad (2566)$$

$$\tau^4_{\gamma,\delta,w,i} = \sum_{\epsilon \in A} Y^2_{i,\epsilon} Z_{\epsilon,\gamma} \tau^3_{\epsilon,\delta,w} \quad (3r_D r_T^3 N_o) \quad (2580)$$

$$\tau^5_{\gamma,\alpha} = \sum_{a \in V} W^2_{a,\alpha} Y^3_{a,\gamma} \quad (2r_T r_V N_v) \quad (2567)$$

$$\tau^5_{\gamma,\delta,\alpha,w} = \sum_{i \in O} W^3_{i,\alpha} \tau^4_{\gamma,\delta,w,i} \quad (2r_D r_T^2 r_V N_o) \quad (2581)$$

$$\tau^6_{\gamma,\alpha,i} = \sum_{\beta \in B} W^1_{i,\beta} X_{\beta,\alpha} \tau^5_{\gamma,\beta} \quad (3r_T r_V^2 N_o) \quad (2568)$$

$$\tau^6_{\gamma,\alpha} = \sum_{a \in V} W^4_{a,\alpha} Y^3_{a,\gamma} \quad (2r_T r_V N_v) \quad (2582)$$

$$\tau^7_{\gamma,\alpha} = \sum_{i \in O} W^3_{i,\alpha} Y^4_{i,\gamma} \quad (2r_T r_V N_o) \quad (2569)$$

$$\tau^7_{\gamma,\alpha,i} = \sum_{\delta \in A} Z_{\gamma,\delta} Y^4_{i,\delta} \tau^6_{\delta,\alpha} \quad (3r_T^2 r_V N_o) \quad (2583)$$

$$\tau^8_{\gamma,\alpha} = \sum_{\delta \in A} \sum_{i \in O} Y^2_{i,\gamma} Z_{\gamma,\delta} \tau^7_{\delta,\alpha} \tau^6_{\delta,\alpha,i} \quad (4r_T^2 r_V N_o) \quad (2570)$$

$$\tau^8_{\gamma,\delta,\alpha,w} = \sum_{i \in O} {}^2D^4_{i,w} Y^{4,*}_{i,\delta} \tau^7_{\gamma,\alpha,i} \quad (3r_D r_T^2 r_V N_o) \quad (2584)$$

$$\tau^9_{\gamma,a} = \sum_{\alpha \in B} W^4_{a,\alpha} \tau^8_{\gamma,\alpha} \quad (2r_T r_V N_v) \quad (2571)$$

$$\tau_{\gamma,\delta,\epsilon,w}^9 = \sum_{\alpha \in B} \tau_{\gamma,\delta,\alpha}^2 \tau_{\delta,\epsilon,\alpha,w}^5 \tau_{\gamma,\epsilon,\alpha,w}^8 \quad (3r_D r_T^3 r_V) \quad (2585)$$

$$\tau_{\gamma,\alpha,w}^7 = \sum_{\delta \in A} \sum_{i \in O} {}^2D_{i,w}^4 Y_{i,\gamma}^{4,*} \tau_{\delta,\alpha}^4 \tau_{\delta,\gamma,w}^3 \tau_{\delta,\alpha,i}^6 \quad (5r_D r_T^2 r_V N_o) \quad (2597)$$

$$\tau_{\gamma,\delta,w,i}^{10} = \sum_{\epsilon \in A} {}^2D_{i,w}^2 Y_{i,\epsilon}^4 \tau_{\gamma,\epsilon,\delta,w}^9 \quad (3r_D r_T^3 N_o) \quad (2586)$$

$$\tau_{\gamma,\alpha,w}^8 = \sum_{\beta \in B} X_{\alpha,\beta} \tau_{\gamma,\beta,w}^7 \quad (2r_D r_T r_V^2) \quad (2598)$$

$$\tau_{\gamma,\delta,w}^{11} = \sum_{\epsilon \in A} \sum_{i \in O} Y_{i,\delta}^{2,*} Z_{\delta,\epsilon}^* \tau_{\gamma,\epsilon,w,i}^{10} \quad (3r_D r_T^3 N_o) \quad (2587)$$

$$\tau_{\gamma,\alpha,w}^9 = \sum_{\delta \in A} Z_{\gamma,\delta}^* \tau_{\delta,\alpha,w}^8 \quad (2r_D r_T^2 r_V) \quad (2599)$$

$$\tau_{\gamma,\delta,w,i}^{10} = \sum_{\alpha \in B} \tau_{\gamma,\alpha}^0 \tau_{\gamma,\alpha,i}^2 \tau_{\delta,\alpha,w}^9 \quad (3r_D r_T^2 r_V N_o) \quad (2600)$$

$${}^{21}R_{a,\gamma} \leftarrow \sum_{\delta \in A} \sum_{w \in D} \frac{1}{4} {}^2D_{a,w}^1 Y_{a,\delta}^1 \tau_{\delta,\gamma,w}^{11} \quad (3r_D r_T^2 N_v) \quad (2588)$$

$$\tau_{\gamma,\delta,w}^{11} = \sum_{i \in O} {}^2D_{i,w}^2 Y_{i,\delta}^{2,*} \tau_{\gamma,\delta,w,i}^{10} \quad (3r_D r_T^2 N_o) \quad (2601)$$

$${}^{21}R_{a,\epsilon} \leftarrow \sum_{\gamma \in A} \sum_{i \in O} \sum_{j \in O} \sum_{k \in O} \sum_{l \in O} \sum_{b \in V} \sum_{c \in V} \sum_{d \in V} \frac{1}{4} Y_{i,\epsilon}^{2,*} Z_{\epsilon,\gamma}^* Y_{b,\gamma}^{3,*} Y_{j,\gamma}^{4,*} {}^2D_{a,i,b,j} {}^2T_{a,i,c,k} {}^2T_{d,j,b,l} V_{k,d,l,c} \quad (2589)$$

$${}^{21}R_{a,\gamma} \leftarrow \sum_{\delta \in A} \sum_{w \in D} \frac{1}{4} {}^2D_{a,w}^1 Y_{a,\delta}^1 \tau_{\delta,\gamma,w}^{11} \quad (3r_D r_T^2 N_v) \quad (2602)$$

Factorized expression

Raw expression

$$\tau_{\gamma,\alpha}^0 = \sum_{i \in O} W_{i,\alpha}^1 Y_{i,\gamma}^2 \quad (2r_T r_V N_o) \quad (2590)$$

$${}^{21}R_{a,\epsilon} \leftarrow \sum_{\gamma \in A} \sum_{i \in O} \sum_{j \in O} \sum_{k \in O} \sum_{l \in O} \sum_{b \in V} \sum_{c \in V} \sum_{d \in V} \frac{1}{4} Y_{i,\epsilon}^{2,*} Z_{\epsilon,\gamma}^* Y_{b,\gamma}^{3,*} Y_{j,\gamma}^{4,*} {}^2D_{a,i,b,j} {}^2T_{a,k,b,j} {}^2T_{c,i,d,l} V_{k,d,l,c} \quad (2603)$$

$$\tau_{\gamma,\alpha}^1 = \sum_{a \in V} W_{a,\alpha}^2 Y_{a,\gamma}^3 \quad (2r_T r_V N_v) \quad (2591)$$

Factorized expression

$$\tau_{\gamma,\alpha,i}^2 = \sum_{\delta \in A} Z_{\gamma,\delta} Y_{i,\delta}^4 \tau_{\delta,\alpha}^1 \quad (3r_T^2 r_V N_o) \quad (2592)$$

$$\tau_{\gamma,\delta,w}^0 = \sum_{i \in O} {}^2D_{i,w}^2 Y_{i,\gamma}^2 Y_{i,\delta}^{2,*} \quad (3r_D r_T^2 N_o) \quad (2604)$$

$$\tau_{\gamma,\delta,w}^3 = \sum_{a \in V} {}^2D_{a,w}^3 Y_{a,\gamma}^1 Y_{a,\delta}^{3,*} \quad (3r_D r_T^2 N_v) \quad (2593)$$

$$\tau_{\gamma,\delta,w}^1 = \sum_{a \in V} {}^2D_{a,w}^3 Y_{a,\gamma}^3 Y_{a,\delta}^{3,*} \quad (3r_D r_T^2 N_v) \quad (2605)$$

$$\tau_{\gamma,\alpha}^4 = \sum_{i \in O} W_{i,\alpha}^3 Y_{i,\gamma}^2 \quad (2r_T r_V N_o) \quad (2594)$$

$$\tau_{\gamma,\alpha}^2 = \sum_{a \in V} W_{a,\alpha}^4 Y_{a,\gamma}^3 \quad (2r_T r_V N_v) \quad (2606)$$

$$\tau_{\gamma,\alpha}^5 = \sum_{a \in V} W_{a,\alpha}^4 Y_{a,\gamma}^3 \quad (2r_T r_V N_v) \quad (2595)$$

$$\tau_{\gamma,\alpha,i}^3 = \sum_{\beta \in B} X_{\alpha,\beta} W_{i,\beta}^3 \tau_{\gamma,\beta}^2 \quad (3r_T r_V^2 N_o) \quad (2607)$$

$$\tau_{\gamma,\alpha,i}^6 = \sum_{\delta \in A} Z_{\gamma,\delta} Y_{i,\delta}^4 \tau_{\delta,\alpha}^5 \quad (3r_T^2 r_V N_o) \quad (2596)$$

$$\tau_{\gamma,\alpha}^4 = \sum_{i \in O} W_{i,\alpha}^1 Y_{i,\gamma}^4 \quad (2r_T r_V N_o) \quad (2608)$$

$$\tau^5_{\gamma,\alpha} = \sum_{a \in V} W^2_{a,\alpha} Y^1_{a,\gamma} \quad (2r_T r_V N_v) \quad (2609)$$

$$\tau^4_{\gamma,\alpha} = \sum_{i \in O} W^3_{i,\alpha} Y^2_{i,\gamma} \quad (2r_T r_V N_o) \quad (2622)$$

$$\tau^6_{\gamma,\delta,i} = \sum_{\alpha \in B} \tau^4_{\delta,\alpha} \tau^5_{\gamma,\alpha} \tau^3_{\delta,\alpha,i} \quad (3r_T^2 r_V N_o) \quad (2610)$$

$$\tau^5_{\gamma,\alpha} = \sum_{a \in V} W^4_{a,\alpha} Y^3_{a,\gamma} \quad (2r_T r_V N_v) \quad (2623)$$

$$\tau^7_{\gamma,\delta,\epsilon} = \sum_{i \in O} Z_{\gamma,\delta} Y^4_{i,\delta} \tau^6_{\gamma,\epsilon,i} \quad (3r_T^3 N_o) \quad (2611)$$

$$\tau^6_{\gamma,\delta,i} = \sum_{\alpha \in B} \tau^4_{\gamma,\alpha} \tau^5_{\delta,\alpha} \tau^3_{\gamma,\alpha,i} \quad (3r_T^2 r_V N_o) \quad (2624)$$

$$\tau^8_{\gamma,\delta,i} = \sum_{\epsilon \in A} Y^2_{i,\epsilon} \tau^7_{\epsilon,\gamma,\delta} \quad (2r_T^3 N_o) \quad (2612)$$

$$\tau^7_{\gamma,i} = \sum_{\delta \in A} Z_{\delta,\gamma} \tau^6_{\delta,\gamma,i} \quad (2r_T^2 N_o) \quad (2625)$$

$$\tau^9_{\gamma,\delta,w} = \sum_{\epsilon \in A} \sum_{i \in O} {}^2D^4_{i,w} Y^{4,*}_{i,\delta} \tau^1_{\epsilon,\delta,w} \tau^8_{\epsilon,\gamma,i} \quad (4r_D r_T^3 N_o) \quad (2613)$$

$$\tau^8_{i,j} = \sum_{\gamma \in A} Y^4_{j,\gamma} \tau^7_{\gamma,i} \quad (2r_T N_o^2) \quad (2626)$$

$$\tau^{10}_{\gamma,\delta,w} = \sum_{\epsilon \in A} Z^*_{\delta,\epsilon} \tau^9_{\gamma,\epsilon,w} \quad (2r_D r_T^3) \quad (2614)$$

$$\tau^9_{\gamma,i} = \sum_{j \in O} Y^4_{j,\gamma} \tau^8_{j,i} \quad (2r_T N_o^2) \quad (2627)$$

$$\tau^{11}_{\gamma,\delta,w} = \sum_{\epsilon \in A} Z_{\gamma,\epsilon} \tau^{10}_{\epsilon,\delta,w} \quad (2r_D r_T^3) \quad (2615)$$

$$\tau^{10}_{\gamma,\delta,w} = \sum_{i \in O} {}^2D^4_{i,w} Y^{4,*}_{i,\delta} \tau^9_{\gamma,i} \quad (3r_D r_T^2 N_o) \quad (2628)$$

$${}^{21}R_{a,\gamma} \leftarrow \sum_{\delta \in A} \sum_{w \in D} \frac{1}{4} {}^2D^1_{a,w} Y^1_{a,\delta} \tau^0_{\delta,\gamma,w} \tau^{11}_{\delta,\gamma,w} \quad (4r_D r_T^2 N_v) \quad (2616)$$

$$\tau^{11}_{\gamma,\delta,w} = \sum_{\epsilon \in A} Z^*_{\delta,\epsilon} \tau^1_{\gamma,\epsilon,w} \tau^{10}_{\gamma,\epsilon,w} \quad (3r_D r_T^3) \quad (2629)$$

Raw expression

$$\tau^{12}_{\gamma,\delta,w} = \sum_{\epsilon \in A} Z_{\gamma,\epsilon} \tau^{11}_{\epsilon,\delta,w} \quad (2r_D r_T^3) \quad (2630)$$

$${}^{21}R_{a,\epsilon} \leftarrow \sum_{\gamma \in A} \sum_{i \in O} \sum_{j \in O} \sum_{k \in O} \sum_{l \in O} \sum_{b \in V} \sum_{c \in V} \sum_{d \in V} \frac{1}{4} Y^{2,*}_{i,\epsilon} Z^*_{\epsilon,\gamma} Y^{3,*}_{b,\gamma} Y^{4,*}_{j,\gamma} {}^2D^{a,i,b,j}_{a,k,b,j} {}^2T_{a,k,b,j} {}^2T_{c,l,d,i} V_{k,c,l,d} \quad (2617)$$

$${}^{21}R_{a,\gamma} \leftarrow \sum_{\delta \in A} \sum_{w \in D} \frac{1}{4} {}^2D^1_{a,w} Y^1_{a,\delta} \tau^0_{\delta,\gamma,w} \tau^{12}_{\delta,\gamma,w} \quad (4r_D r_T^2 N_v) \quad (2631)$$

Factorized expression

Raw expression

$$\tau^0_{\gamma,\delta,w} = \sum_{i \in O} {}^2D^2_{i,w} Y^2_{i,\gamma} Y^{2,*}_{i,\delta} \quad (3r_D r_T^2 N_o) \quad (2618)$$

$${}^{21}R_{a,\epsilon} \leftarrow \sum_{\gamma \in A} \sum_{i \in O} \sum_{j \in O} \sum_{k \in O} \sum_{l \in O} \sum_{b \in V} \sum_{c \in V} \sum_{d \in V} \frac{1}{4} Y^{2,*}_{i,\epsilon} Z^*_{\epsilon,\gamma} Y^{3,*}_{b,\gamma} Y^{4,*}_{j,\gamma} {}^2D^{a,i,b,j}_{a,k,b,l} {}^2T_{a,k,b,l} {}^2T_{c,i,d,j} V_{k,c,l,d} \quad (2632)$$

$$\tau^1_{\gamma,\delta,w} = \sum_{a \in V} {}^2D^3_{a,w} Y^3_{a,\gamma} Y^{3,*}_{a,\delta} \quad (3r_D r_T^2 N_v) \quad (2619)$$

Factorized expression

$$\tau^2_{\gamma,\alpha} = \sum_{a \in V} W^2_{a,\alpha} Y^1_{a,\gamma} \quad (2r_T r_V N_v) \quad (2620)$$

$$\tau^0_{\gamma,\delta,w} = \sum_{a \in V} {}^2D^3_{a,w} Y^3_{a,\gamma} Y^{3,*}_{a,\delta} \quad (3r_D r_T^2 N_v) \quad (2633)$$

$$\tau^3_{\gamma,\alpha,i} = \sum_{\beta \in B} W^1_{i,\beta} X_{\beta,\alpha} \tau^2_{\gamma,\beta} \quad (3r_T r_V^2 N_o) \quad (2621)$$

$$\tau^1_{\gamma,\delta,w,i} = \sum_{\epsilon \in A} Z_{\gamma,\epsilon} Y^4_{i,\epsilon} \tau^0_{\epsilon,\delta,w} \quad (3r_D r_T^3 N_o) \quad (2634)$$



$$\tau^2_{\gamma,\delta,\alpha,w} = \sum_{i \in O} W^3_{i,\alpha} \tau^1_{\gamma,\delta,w,i} \quad (2r_D r_T^2 r_V N_o) \quad (2635)$$

$$\tau^0_{\gamma,\delta,w} = \sum_{a \in V} {}^2D^3_{a,w} Y^3_{a,\gamma} Y^{3,*}_{a,\delta} \quad (3r_D r_T^2 N_v) \quad (2647)$$

$$\tau^3_{\gamma,\alpha} = \sum_{a \in V} W^2_{a,\alpha} Y^1_{a,\gamma} \quad (2r_T r_V N_v) \quad (2636)$$

$$\tau^1_{\gamma,\delta,w,i} = \sum_{\epsilon \in A} Z^*_{\delta,\epsilon} Y^{4,*}_{i,\epsilon} \tau^0_{\gamma,\epsilon,w} \quad (3r_D r_T^3 N_o) \quad (2648)$$

$$\tau^4_{\gamma,\alpha,i} = \sum_{\beta \in B} W^1_{i,\beta} X_{\beta,\alpha} \tau^3_{\gamma,\beta} \quad (3r_T r_V^2 N_o) \quad (2637)$$

$$\tau^2_{\gamma,\alpha} = \sum_{a \in V} W^2_{a,\alpha} Y^1_{a,\gamma} \quad (2r_T r_V N_v) \quad (2649)$$

$$\tau^5_{\gamma,\delta,\alpha} = \sum_{i \in O} Y^2_{i,\delta} \tau^4_{\gamma,\alpha,i} \quad (2r_T^2 r_V N_o) \quad (2638)$$

$$\tau^3_{\gamma,\alpha,i} = \sum_{\beta \in B} W^1_{i,\beta} X_{\beta,\alpha} \tau^2_{\gamma,\beta} \quad (3r_T r_V^2 N_o) \quad (2650)$$

$$\tau^6_{\gamma,\alpha} = \sum_{a \in V} W^4_{a,\alpha} Y^3_{a,\gamma} \quad (2r_T r_V N_v) \quad (2639)$$

$$\tau^4_{\gamma,\alpha} = \sum_{a \in V} W^4_{a,\alpha} Y^3_{a,\gamma} \quad (2r_T r_V N_v) \quad (2651)$$

$$\tau^7_{\gamma,\alpha,i} = \sum_{\delta \in A} Z_{\gamma,\delta} Y^4_{i,\delta} \tau^6_{\delta,\alpha} \quad (3r_T^2 r_V N_o) \quad (2640)$$

$$\tau^5_{\gamma,\alpha,i} = \sum_{\delta \in A} Z_{\gamma,\delta} Y^4_{i,\delta} \tau^4_{\delta,\alpha} \quad (3r_T^2 r_V N_o) \quad (2652)$$

$$\tau^8_{\gamma,\delta,\alpha,w} = \sum_{i \in O} {}^2D^4_{i,w} Y^{4,*}_{i,\delta} \tau^7_{\gamma,\alpha,i} \quad (3r_D r_T^2 r_V N_o) \quad (2641)$$

$$\tau^6_{\gamma,i,j,k} = \sum_{\alpha \in B} W^3_{j,\alpha} \tau^3_{\gamma,\alpha,i} \tau^5_{\gamma,\alpha,k} \quad (3r_T r_V N_o^3) \quad (2653)$$

$$\tau^9_{\gamma,\delta,\epsilon,w} = \sum_{\alpha \in B} \tau^5_{\gamma,\delta,\alpha} \tau^2_{\gamma,\epsilon,\alpha,w} \tau^8_{\delta,\epsilon,\alpha,w} \quad (3r_D r_T^3 r_V) \quad (2642)$$

$$\tau^7_{i,j,k,l} = \sum_{\gamma \in A} Y^2_{k,\gamma} \tau^6_{\gamma,i,j,l} \quad (2r_T N_o^4) \quad (2654)$$

$$\tau^{10}_{\gamma,\delta,w,i} = \sum_{\epsilon \in A} {}^2D^2_{i,w} Y^2_{i,\epsilon} \tau^9_{\epsilon,\gamma,\delta,w} \quad (3r_D r_T^3 N_o) \quad (2643)$$

$$\tau^8_{\gamma,i,j,k} = \sum_{l \in O} Y^4_{l,\gamma} \tau^7_{i,l,j,k} \quad (2r_T N_o^4) \quad (2655)$$

$$\tau^9_{\gamma,\delta,w,i} = \sum_{j \in O} \sum_{k \in O} {}^2D^2_{j,w} {}^2D^4_{k,w} Y^{2,*}_{j,\delta} \tau^1_{\gamma,\delta,w,k} \tau^8_{\gamma,i,j,k} \quad (5r_D r_T^2 N_o) \quad (2656)$$

$$\tau^{11}_{\gamma,\delta,w} = \sum_{\epsilon \in A} \sum_{i \in O} Y^{2,*}_{i,\delta} Z^*_{\delta,\epsilon} \tau^{10}_{\gamma,\epsilon,w,i} \quad (3r_D r_T^3 N_o) \quad (2644)$$

$$\tau^{10}_{\gamma,\delta,w} = \sum_{\epsilon \in A} \sum_{i \in O} Y^2_{i,\gamma} Z_{\gamma,\epsilon} \tau^9_{\epsilon,\delta,w,i} \quad (3r_D r_T^3 N_o) \quad (2657)$$

$${}^{21}R_{a,\gamma} \leftarrow \sum_{\delta \in A} \sum_{w \in D} \frac{1}{4} {}^2D^1_{a,w} Y^1_{a,\delta} \tau^{11}_{\delta,\gamma,w} \quad (3r_D r_T^2 N_v) \quad (2645)$$

$${}^{21}R_{a,\gamma} \leftarrow \sum_{\delta \in A} \sum_{w \in D} \frac{1}{4} {}^2D^1_{a,w} Y^1_{a,\delta} \tau^{10}_{\delta,\gamma,w} \quad (3r_D r_T^2 N_v) \quad (2658)$$

Raw expression

Raw expression

$${}^{21}R_{a,\epsilon} \leftarrow \sum_{\gamma \in A} \sum_{i \in O} \sum_{j \in O} \sum_{k \in O} \sum_{l \in O} \sum_{b \in V} \sum_{c \in V} \sum_{d \in V} \frac{1}{4} Y^{2,*}_{i,\epsilon} Z^*_{\epsilon,\gamma} Y^{3,*}_{b,\gamma} Y^{4,*}_{j,\gamma} {}^2D^{a,i,b,j} {}^2T_{a,k,b,l} {}^2T_{c,j,d,i} V_{k,d,l,c} \quad (2646)$$

$${}^{21}R_{a,\epsilon} \leftarrow \sum_{\gamma \in A} \sum_{i \in O} \sum_{j \in O} \sum_{k \in O} \sum_{l \in O} \sum_{b \in V} \sum_{c \in V} \sum_{d \in V} \frac{1}{4} Y^{2,*}_{i,\epsilon} Z^*_{\epsilon,\gamma} Y^{3,*}_{b,\gamma} Y^{4,*}_{j,\gamma} {}^2D^{a,i,b,j} {}^2T_{a,k,c,i} {}^2T_{b,j,d,l} V_{k,d,l,c} \quad (2659)$$

Factorized expression

Factorized expression

$$\tau^0_{\gamma,\delta,w} = \sum_{a \in V} {}^2D^3_{a,w} Y^3_{a,\gamma} Y^{3,*}_{a,\delta} \quad (3r_D r_T^2 N_v) \quad (2660)$$

$$\tau^1_{\gamma,\delta,w} = \sum_{i \in O} {}^2D^4_{i,w} Y^4_{i,\gamma} Y^{4,*}_{i,\delta} \quad (3r_D r_T^2 N_o) \quad (2661)$$

$$\tau^2_{\gamma,\delta,w} = \sum_{\epsilon \in A} Z^*_{\delta,\epsilon} \tau^0_{\gamma,\epsilon,w} \tau^1_{\gamma,\epsilon,w} \quad (3r_D r_T^3) \quad (2662)$$

$$\tau^3_{\gamma,\delta,w} = \sum_{\epsilon \in A} Z_{\gamma,\epsilon} \tau^2_{\epsilon,\delta,w} \quad (2r_D r_T^3) \quad (2663)$$

$$\tau^4_{\gamma,\alpha} = \sum_{a \in V} W^2_{a,\alpha} Y^1_{a,\gamma} \quad (2r_T r_V N_v) \quad (2664)$$

$$\tau^5_{\gamma,\alpha,i} = \sum_{\beta \in B} W^1_{i,\beta} X_{\beta,\alpha} \tau^4_{\gamma,\beta} \quad (3r_T r_V^2 N_o) \quad (2665)$$

$$\tau^6_{\gamma,\alpha} = \sum_{i \in O} W^3_{i,\alpha} Y^2_{i,\gamma} \quad (2r_T r_V N_o) \quad (2666)$$

$$\tau^7_{\gamma,\alpha} = \sum_{a \in V} W^4_{a,\alpha} Y^3_{a,\gamma} \quad (2r_T r_V N_v) \quad (2667)$$

$$\tau^8_{\gamma,\delta,i} = \sum_{\alpha \in B} \tau^6_{\gamma,\alpha} \tau^7_{\delta,\alpha} \tau^5_{\gamma,\alpha,i} \quad (3r_T^2 r_V N_o) \quad (2668)$$

$$\tau^9_{\gamma,\delta,\epsilon} = \sum_{i \in O} Y^2_{i,\delta} Z_{\delta,\epsilon} \tau^8_{\gamma,\epsilon,i} \quad (3r_T^3 N_o) \quad (2669)$$

$$\tau^{10}_{\gamma,\delta,i} = \sum_{\epsilon \in A} Y^4_{i,\epsilon} \tau^9_{\gamma,\delta,\epsilon} \quad (2r_T^3 N_o) \quad (2670)$$

$$\tau^{11}_{\gamma,\delta,w} = \sum_{\epsilon \in A} \sum_{i \in O} {}^2D^2_{i,w} Y^{2,*}_{i,\delta} \tau^{10}_{\epsilon,\gamma,i} \tau^3_{\epsilon,\delta,w} \quad (4r_D r_T^3 N_o) \quad (2671)$$

$${}^{21}R_{a,\gamma} \leftarrow \sum_{\delta \in A} \sum_{w \in D} \frac{1}{4} {}^2D^1_{a,w} Y^1_{a,\gamma} \tau^{11}_{\delta,\gamma,w} \quad (3r_D r_T^2 N_v) \quad (2672)$$

Raw expression

$${}^{21}R_{a,\epsilon} \leftarrow \sum_{\gamma \in A} \sum_{i \in O} \sum_{j \in O} \sum_{k \in O} \sum_{l \in O} \sum_{b \in V} \sum_{c \in V} \sum_{d \in V} \frac{1}{4} Y^{2,*}_{i,\epsilon} Z^*_{\epsilon,\gamma} Y^{3,*}_{b,\gamma} Y^{4,*}_{j,\gamma} {}^2D^{a,i,b,j}_{a,\gamma} {}^2T_{a,k,c,i} {}^2T_{b,l,d,j} V_{k,c,l,d} \quad (2673)$$

Factorized expression

$$\tau^0_{\gamma,\alpha} = \sum_{a \in V} W^2_{a,\alpha} Y^1_{a,\gamma} \quad (2r_T r_V N_v) \quad (2674)$$

$$\tau^1_{\gamma,\alpha,i} = \sum_{\beta \in B} W^1_{i,\beta} X_{\beta,\alpha} \tau^0_{\gamma,\beta} \quad (3r_T r_V^2 N_o) \quad (2675)$$

$$\tau^2_{\gamma,\alpha} = \sum_{i \in O} W^3_{i,\alpha} Y^2_{i,\gamma} \quad (2r_T r_V N_o) \quad (2676)$$

$$\tau^3_{\gamma,\alpha} = \sum_{a \in V} W^4_{a,\alpha} Y^3_{a,\gamma} \quad (2r_T r_V N_v) \quad (2677)$$

$$\tau^4_{\gamma,\delta,i} = \sum_{\alpha \in B} \tau^2_{\gamma,\alpha} \tau^3_{\delta,\alpha} \tau^1_{\gamma,\alpha,i} \quad (3r_T^2 r_V N_o) \quad (2678)$$

$$\tau^5_{\gamma,i} = \sum_{\delta \in A} Z_{\delta,\gamma} \tau^4_{\delta,\gamma,i} \quad (2r_T^2 N_o) \quad (2679)$$

$$\tau^6_{i,j} = \sum_{\gamma \in A} Y^4_{j,\gamma} \tau^5_{\gamma,i} \quad (2r_T N_o^2) \quad (2680)$$

$$\tau^7_{\gamma,i} = \sum_{j \in O} Y^2_{j,\gamma} \tau^6_{j,i} \quad (2r_T N_o^2) \quad (2681)$$

$$\tau^8_{\gamma,\delta,w} = \sum_{i \in O} {}^2D^2_{i,w} Y^{2,*}_{i,\delta} \tau^7_{\gamma,i} \quad (3r_D r_T^2 N_o) \quad (2682)$$

$$\tau^9_{\gamma,\delta,w} = \sum_{a \in V} {}^2D^3_{a,w} Y^3_{a,\gamma} Y^{3,*}_{a,\delta} \quad (3r_D r_T^2 N_v) \quad (2683)$$

$$\tau^{10}_{\gamma,\delta,w} = \sum_{i \in O} {}^2D^4_{i,w} Y^4_{i,\gamma} Y^{4,*}_{i,\delta} \quad (3r_D r_T^2 N_o) \quad (2684)$$

$$\tau^{11}_{\gamma,\delta,w} = \sum_{\epsilon \in A} Z^*_{\delta,\epsilon} \tau^{10}_{\gamma,\epsilon,w} \tau^9_{\gamma,\epsilon,w} \quad (3r_D r_T^3) \quad (2685)$$

$$\tau^{12}_{\gamma,\delta,w} = \sum_{\epsilon \in A} Z_{\gamma,\epsilon} \tau^{11}_{\epsilon,\delta,w} \quad (2r_D r_T^3) \quad (2686)$$

$${}^{21}R_{a,\gamma} \leftarrow \sum_{\delta \in A} \sum_{w \in D} \frac{1}{4} {}^2D^1_{a,w} Y^1_{a,\delta} \tau^{12}_{\delta,\gamma,w} \tau^8_{\delta,\gamma,w} \quad (4r_D r_T^2 N_v) \quad \tau^{11}_{\gamma,\delta,w} = \sum_{\epsilon \in A} Z^*_{\delta,\epsilon} \tau^1_{\gamma,\epsilon,w} \tau^{10}_{\gamma,\epsilon,w} \quad (3r_D r_T^3) \quad (2700)$$

$$(2687)$$

Raw expression

$$\tau^{12}_{\gamma,\delta,w} = \sum_{\epsilon \in A} Z_{\gamma,\epsilon} \tau^{11}_{\epsilon,\delta,w} \quad (2r_D r_T^3) \quad (2701)$$

$${}^{21}R_{a,\epsilon} \leftarrow \sum_{\gamma \in A} \sum_{i \in O} \sum_{j \in O} \sum_{k \in O} \sum_{l \in O} \sum_{b \in V} \sum_{c \in V} \sum_{d \in V} \frac{1}{4} Y^{2,*}_{i,\epsilon} Z^*_{\epsilon,\gamma} Y^{3,*}_{b,\gamma} Y^{4,*}_{j,\gamma} {}^2D^{a,i,b,j}_{a,\gamma} {}^2T_{a,k,c,i} {}^2T_{d,j,b,l} V_{k,c,l,d} \quad (2688)$$

$${}^{21}R_{a,\gamma} \leftarrow \sum_{\delta \in A} \sum_{w \in D} \frac{1}{4} {}^2D^1_{a,w} Y^1_{a,\delta} \tau^0_{\delta,\gamma,w} \tau^{12}_{\delta,\gamma,w} \quad (4r_D r_T^2 N_v) \quad (2702)$$

Factorized expression

Raw expression

$$\tau^0_{\gamma,\delta,w} = \sum_{i \in O} {}^2D^2_{i,w} Y^2_{i,\gamma} Y^{2,*}_{i,\delta} \quad (3r_D r_T^2 N_o) \quad (2689)$$

$${}^{21}R_{a,\epsilon} \leftarrow \sum_{\gamma \in A} \sum_{i \in O} \sum_{j \in O} \sum_{k \in O} \sum_{l \in O} \sum_{b \in V} \sum_{c \in V} \sum_{d \in V} \frac{1}{4} Y^{2,*}_{i,\epsilon} Z^*_{\epsilon,\gamma} Y^{3,*}_{b,\gamma} Y^{4,*}_{j,\gamma} {}^2D^{a,i,b,j}_{a,\gamma} {}^2T_{a,k,c,i} {}^2T_{d,l,b,j} V_{k,d,l,c} \quad (2703)$$

$$\tau^1_{\gamma,\delta,w} = \sum_{a \in V} {}^2D^3_{a,w} Y^3_{a,\gamma} Y^{3,*}_{a,\delta} \quad (3r_D r_T^2 N_v) \quad (2690)$$

Factorized expression

$$\tau^2_{\gamma,\alpha} = \sum_{a \in V} W^2_{a,\alpha} Y^3_{a,\gamma} \quad (2r_T r_V N_v) \quad (2691)$$

$$\tau^0_{\gamma,\delta,w} = \sum_{i \in O} {}^2D^2_{i,w} Y^2_{i,\gamma} Y^{2,*}_{i,\delta} \quad (3r_D r_T^2 N_o) \quad (2704)$$

$$\tau^3_{\gamma,\alpha,i} = \sum_{\beta \in B} W^1_{i,\beta} X_{\beta,\alpha} \tau^2_{\gamma,\beta} \quad (3r_T r_V^2 N_o) \quad (2692)$$

$$\tau^1_{\gamma,\alpha} = \sum_{a \in V} W^4_{a,\alpha} Y^1_{a,\gamma} \quad (2r_T r_V N_v) \quad (2705)$$

$$\tau^4_{\gamma,\alpha} = \sum_{i \in O} W^3_{i,\alpha} Y^4_{i,\gamma} \quad (2r_T r_V N_o) \quad (2693)$$

$$\tau^2_{\gamma,\alpha,i} = \sum_{\beta \in B} X_{\alpha,\beta} W^3_{i,\beta} \tau^1_{\gamma,\beta} \quad (3r_T r_V^2 N_o) \quad (2706)$$

$$\tau^5_{\gamma,\alpha} = \sum_{a \in V} W^4_{a,\alpha} Y^1_{a,\gamma} \quad (2r_T r_V N_v) \quad (2694)$$

$$\tau^3_{\gamma,\alpha} = \sum_{i \in O} W^1_{i,\alpha} Y^2_{i,\gamma} \quad (2r_T r_V N_o) \quad (2707)$$

$$\tau^6_{\gamma,\delta,i} = \sum_{\alpha \in B} \tau^4_{\delta,\alpha} \tau^5_{\gamma,\alpha} \tau^3_{\delta,\alpha,i} \quad (3r_T^2 r_V N_o) \quad (2695)$$

$$\tau^4_{\gamma,\alpha} = \sum_{\delta \in A} \sum_{i \in O} Z_{\delta,\gamma} Y^4_{i,\gamma} \tau^3_{\delta,\alpha} \tau^2_{\delta,\alpha,i} \quad (4r_T^2 r_V N_o) \quad (2708)$$

$$\tau^7_{\gamma,i} = \sum_{\delta \in A} Z_{\gamma,\delta} \tau^6_{\gamma,\delta,i} \quad (2r_T^2 N_o) \quad (2696)$$

$$\tau^5_{\gamma,a} = \sum_{\alpha \in B} W^2_{a,\alpha} \tau^4_{\gamma,\alpha} \quad (2r_T r_V N_v) \quad (2709)$$

$$\tau^8_{i,j} = \sum_{\gamma \in A} Y^2_{j,\gamma} \tau^7_{\gamma,i} \quad (2r_T N_o^2) \quad (2697)$$

$$\tau^6_{a,b} = \sum_{\gamma \in A} Y^3_{b,\gamma} \tau^5_{\gamma,a} \quad (2r_T N_v^2) \quad (2710)$$

$$\tau^9_{\gamma,i} = \sum_{j \in O} Y^4_{j,\gamma} \tau^8_{j,i} \quad (2r_T N_o^2) \quad (2698)$$

$$\tau^7_{\gamma,a} = \sum_{b \in V} Y^3_{b,\gamma} \tau^6_{b,a} \quad (2r_T N_v^2) \quad (2711)$$

$$\tau^{10}_{\gamma,\delta,w} = \sum_{i \in O} {}^2D^4_{i,w} Y^{4,*}_{i,\delta} \tau^9_{\gamma,i} \quad (3r_D r_T^2 N_o) \quad (2699)$$

$$\tau^8_{\gamma,\delta,w} = \sum_{a \in V} {}^2D^3_{a,w} Y^{3,*}_{a,\delta} \tau^7_{\gamma,a} \quad (3r_D r_T^2 N_v) \quad (2712)$$

$$\tau^9_{\gamma,\delta,w} = \sum_{i \in O} {}^2D^4_{i,w} Y^4_{i,\gamma} Y^{4,*}_{i,\delta} \quad (3r_D r_T^2 N_o) \quad (2713)$$

$$\tau^{10}_{\gamma,\delta,w} = \sum_{\epsilon \in A} Z^*_{\delta,\epsilon} \tau^8_{\gamma,\epsilon,w} \tau^9_{\gamma,\epsilon,w} \quad (3r_D r_T^3) \quad (2714)$$

$$\tau^{11}_{\gamma,\delta,w} = \sum_{\epsilon \in A} Z_{\gamma,\epsilon} \tau^{10}_{\epsilon,\delta,w} \quad (2r_D r_T^3) \quad (2715)$$

$${}^{21}R_{a,\gamma} \leftarrow \sum_{\delta \in A} \sum_{w \in D} \frac{1}{4} {}^2D^1_{a,w} Y^1_{a,\delta} \tau^0_{\delta,\gamma,w} \tau^{11}_{\delta,\gamma,w} \quad (4r_D r_T^2 N_v) \quad (2716)$$

Raw expression

$${}^{21}R_{a,\epsilon} \leftarrow \sum_{\gamma \in A} \sum_{i \in O} \sum_{j \in O} \sum_{k \in O} \sum_{l \in O} \sum_{b \in V} \sum_{c \in V} \sum_{d \in V} \frac{1}{4} Y^{2,*}_{i,\epsilon} Z^*_{\epsilon,\gamma} Y^{3,*}_{b,\gamma} Y^{4,*}_{j,\gamma} {}^2D^{a,i,b,j} {}^2T_{a,k,c,j} {}^2T_{b,l,d,i} V_{k,d,l,c} \quad (2717)$$

Factorized expression

$$\tau^0_{\gamma,\delta,w} = \sum_{i \in O} {}^2D^2_{i,w} Y^2_{i,\gamma} Y^{2,*}_{i,\delta} \quad (3r_D r_T^2 N_o) \quad (2718)$$

$$\tau^1_{\gamma,\delta,w} = \sum_{a \in V} {}^2D^3_{a,w} Y^3_{a,\gamma} Y^{3,*}_{a,\delta} \quad (3r_D r_T^2 N_v) \quad (2719)$$

$$\tau^2_{\gamma,\delta,w} = \sum_{i \in O} {}^2D^4_{i,w} Y^4_{i,\gamma} Y^{4,*}_{i,\delta} \quad (3r_D r_T^2 N_o) \quad (2720)$$

$$\tau^3_{\gamma,\delta,w} = \sum_{\epsilon \in A} Z^*_{\delta,\epsilon} \tau^1_{\gamma,\epsilon,w} \tau^2_{\gamma,\epsilon,w} \quad (3r_D r_T^3) \quad (2721)$$

$$\tau^4_{\gamma,\delta,w} = \sum_{\epsilon \in A} Z_{\gamma,\epsilon} \tau^3_{\epsilon,\delta,w} \quad (2r_D r_T^3) \quad (2722)$$

$$\tau^5_{\gamma,\alpha} = \sum_{a \in V} W^2_{a,\alpha} Y^3_{a,\gamma} \quad (2r_T r_V N_v) \quad (2723)$$

$$\tau^6_{\gamma,\alpha,i} = \sum_{\beta \in B} W^1_{i,\beta} X_{\beta,\alpha} \tau^5_{\gamma,\beta} \quad (3r_T r_V^2 N_o) \quad (2724)$$

$$\tau^7_{\gamma,\alpha} = \sum_{i \in O} W^3_{i,\alpha} Y^4_{i,\gamma} \quad (2r_T r_V N_o) \quad (2725)$$

$$\tau^8_{\gamma,\alpha} = \sum_{\delta \in A} \sum_{i \in O} Y^2_{i,\gamma} Z_{\gamma,\delta} \tau^7_{\delta,\alpha} \tau^6_{\delta,\alpha,i} \quad (4r_T^2 r_V N_o) \quad (2726)$$

$$\tau^9_{\gamma,a} = \sum_{\alpha \in B} W^4_{a,\alpha} \tau^8_{\gamma,\alpha} \quad (2r_T r_V N_v) \quad (2727)$$

$$\tau^{10}_{\gamma,\delta} = \sum_{a \in V} Y^1_{a,\gamma} \tau^9_{\delta,a} \quad (2r_T^2 N_v) \quad (2728)$$

$$\tau^{11}_{\gamma,a} = \sum_{\delta \in A} Y^1_{a,\delta} \tau^{10}_{\gamma,\delta} \quad (2r_T^2 N_v) \quad (2729)$$

$${}^{21}R_{a,\gamma} \leftarrow \sum_{\delta \in A} \sum_{w \in D} \frac{1}{4} {}^2D^1_{a,w} \tau^{11}_{\delta,a} \tau^0_{\delta,\gamma,w} \tau^4_{\delta,\gamma,w} \quad (4r_D r_T^2 N_v) \quad (2730)$$

Raw expression

$${}^{21}R_{a,\epsilon} \leftarrow \sum_{\gamma \in A} \sum_{i \in O} \sum_{j \in O} \sum_{k \in O} \sum_{l \in O} \sum_{b \in V} \sum_{c \in V} \sum_{d \in V} \frac{1}{4} Y^{2,*}_{i,\epsilon} Z^*_{\epsilon,\gamma} Y^{3,*}_{b,\gamma} Y^{4,*}_{j,\gamma} {}^2D^{a,i,b,j} {}^2T_{a,k,c,j} {}^2T_{d,i,b,l} V_{k,d,l,c} \quad (2731)$$

Factorized expression

$$\tau^0_{\gamma,\alpha} = \sum_{a \in V} W^2_{a,\alpha} Y^3_{a,\gamma} \quad (2r_T r_V N_v) \quad (2732)$$

$$\tau^1_{\gamma,\alpha,i} = \sum_{\beta \in B} W^1_{i,\beta} X_{\beta,\alpha} \tau^0_{\gamma,\beta} \quad (3r_T r_V^2 N_o) \quad (2733)$$

$$\tau^2_{\gamma,\alpha} = \sum_{i \in O} W^3_{i,\alpha} Y^4_{i,\gamma} \quad (2r_T r_V N_o) \quad (2734)$$

$$\tau^3_{\gamma,\alpha} = \sum_{a \in V} W^4_{a,\alpha} Y^1_{a,\gamma} \quad (2r_T r_V N_v) \quad (2735)$$

$$\tau^4_{\gamma,\delta,i} = \sum_{\alpha \in B} \tau^2_{\delta,\alpha} \tau^3_{\gamma,\alpha} \tau^1_{\delta,\alpha,i} \quad (3r_T^2 r_V N_o) \quad (2736)$$

$$\tau^5_{\gamma,i} = \sum_{\delta \in A} Z_{\gamma,\delta} \tau^4_{\gamma,\delta,i} \quad (2r_T^2 N_o) \quad (2737)$$

$$\tau^6_{i,j} = \sum_{\gamma \in A} Y^2_{j,\gamma} \tau^5_{\gamma,i} \quad (2r_T N_o^2) \quad (2738)$$

$$\tau^7_{\gamma,i} = \sum_{j \in O} Y^2_{j,\gamma} \tau^6_{j,i} \quad (2r_T N_o^2) \quad (2739)$$

$$\tau^5_{\gamma,\alpha,w} = \sum_{\beta \in B} X_{\alpha,\beta} \tau^4_{\gamma,\beta,w} \quad (2r_D r_T r_V^2) \quad (2752)$$

$$\tau^8_{\gamma,\delta,w} = \sum_{i \in O} {}^2D^2_{i,w} Y^{2,*}_{i,\delta} \tau^7_{\gamma,i} \quad (3r_D r_T^2 N_o) \quad (2740)$$

$$\tau^6_{\gamma,\alpha,w} = \sum_{\delta \in A} Z^*_{\gamma,\delta} \tau^5_{\delta,\alpha,w} \quad (2r_D r_T^2 r_V) \quad (2753)$$

$$\tau^9_{\gamma,\delta,w} = \sum_{a \in V} {}^2D^3_{a,w} Y^3_{a,\gamma} Y^{3,*}_{a,\delta} \quad (3r_D r_T^2 N_v) \quad (2741)$$

$$\tau^7_{\gamma,\alpha} = \sum_{i \in O} W^1_{i,\alpha} Y^2_{i,\gamma} \quad (2r_T r_V N_o) \quad (2754)$$

$$\tau^{10}_{\gamma,\delta,w} = \sum_{i \in O} {}^2D^4_{i,w} Y^4_{i,\gamma} Y^{4,*}_{i,\delta} \quad (3r_D r_T^2 N_o) \quad (2742)$$

$$\tau^8_{\gamma,\alpha} = \sum_{a \in V} W^2_{a,\alpha} Y^3_{a,\gamma} \quad (2r_T r_V N_v) \quad (2755)$$

$$\tau^{11}_{\gamma,\delta,w} = \sum_{\epsilon \in A} Z^*_{\delta,\epsilon} \tau^{10}_{\gamma,\epsilon,w} \tau^9_{\gamma,\epsilon,w} \quad (3r_D r_T^3) \quad (2743)$$

$$\tau^9_{\gamma,\alpha,i} = \sum_{\delta \in A} Z_{\gamma,\delta} Y^4_{i,\delta} \tau^8_{\delta,\alpha} \quad (3r_T^2 r_V N_o) \quad (2756)$$

$$\tau^{12}_{\gamma,\delta,w} = \sum_{\epsilon \in A} Z_{\gamma,\epsilon} \tau^{11}_{\epsilon,\delta,w} \quad (2r_D r_T^3) \quad (2744)$$

$$\tau^{10}_{\gamma,\delta,w,i} = \sum_{\alpha \in B} \tau^7_{\gamma,\alpha} \tau^6_{\delta,\alpha,w} \tau^9_{\gamma,\alpha,i} \quad (3r_D r_T^2 r_V N_o) \quad (2757)$$

$${}^{21}R_{a,\gamma} \leftarrow \sum_{\delta \in A} \sum_{w \in D} \frac{1}{4} {}^2D^1_{a,w} Y^1_{a,\delta} \tau^{12}_{\delta,\gamma,w} \tau^8_{\delta,\gamma,w} \quad (4r_D r_T^2 N_v) \quad (2745)$$

$$\tau^{11}_{\gamma,\delta,w} = \sum_{i \in O} {}^2D^2_{i,w} Y^{2,*}_{i,\delta} \tau^{10}_{\gamma,\delta,w,i} \quad (3r_D r_T^2 N_o) \quad (2758)$$

Raw expression

$${}^{21}R_{a,\epsilon} \leftarrow \sum_{\gamma \in A} \sum_{i \in O} \sum_{j \in O} \sum_{k \in O} \sum_{l \in O} \sum_{b \in V} \sum_{c \in V} \sum_{d \in V} \frac{1}{4} Y^{2,*}_{i,\epsilon} Z^*_{\epsilon,\gamma} Y^{3,*}_{b,\gamma} Y^{4,*}_{j,\gamma} {}^2D^{a,i,b,j}_{a,k,c,l} {}^2T_{b,j,d,i} V_{k,c,l,d} \quad (2746)$$

$${}^{21}R_{a,\gamma} \leftarrow \sum_{\delta \in A} \sum_{w \in D} \frac{1}{4} {}^2D^1_{a,w} Y^1_{a,\delta} \tau^{11}_{\delta,\gamma,w} \quad (3r_D r_T^2 N_v) \quad (2759)$$

Raw expression

Factorized expression

$$\tau^0_{\gamma,\delta,w} = \sum_{a \in V} {}^2D^3_{a,w} Y^3_{a,\gamma} Y^{3,*}_{a,\delta} \quad (3r_D r_T^2 N_v) \quad (2747)$$

$${}^{21}R_{a,\epsilon} \leftarrow \sum_{\gamma \in A} \sum_{i \in O} \sum_{j \in O} \sum_{k \in O} \sum_{l \in O} \sum_{b \in V} \sum_{c \in V} \sum_{d \in V} \frac{1}{4} Y^{2,*}_{i,\epsilon} Z^*_{\epsilon,\gamma} Y^{3,*}_{b,\gamma} Y^{4,*}_{j,\gamma} {}^2D^{a,i,b,j}_{a,k,c,l} {}^2T_{d,i,b,j} V_{k,c,l,d} \quad (2760)$$

Factorized expression

$$\tau^1_{\gamma,\alpha} = \sum_{a \in V} W^4_{a,\alpha} Y^1_{a,\gamma} \quad (2r_T r_V N_v) \quad (2748)$$

$$\tau^0_{\gamma,\delta,w} = \sum_{a \in V} {}^2D^3_{a,w} Y^3_{a,\gamma} Y^{3,*}_{a,\delta} \quad (3r_D r_T^2 N_v) \quad (2761)$$

$$\tau^2_{\gamma,\alpha,i} = \sum_{\delta \in A} Y^2_{i,\delta} Z_{\delta,\gamma} \tau^1_{\delta,\alpha} \quad (3r_T^2 r_V N_o) \quad (2749)$$

$$\tau^1_{\gamma,\delta,w,i} = \sum_{\epsilon \in A} Z^*_{\delta,\epsilon} Y^{4,*}_{i,\epsilon} \tau^0_{\gamma,\epsilon,w} \quad (3r_D r_T^3 N_o) \quad (2762)$$

$$\tau^3_{\gamma,\alpha} = \sum_{i \in O} W^3_{i,\alpha} Y^4_{i,\gamma} \quad (2r_T r_V N_o) \quad (2750)$$

$$\tau^2_{\gamma,\alpha} = \sum_{a \in V} W^4_{a,\alpha} Y^1_{a,\gamma} \quad (2r_T r_V N_v) \quad (2763)$$

$$\tau^4_{\gamma,\alpha,w} = \sum_{\delta \in A} \sum_{i \in O} {}^2D^4_{i,w} Y^{4,*}_{i,\gamma} \tau^3_{\delta,\alpha} \tau^0_{\delta,\gamma,w} \tau^2_{\delta,\alpha,i} \quad (5r_D r_T^2 r_V N_o) \quad (2751)$$

$$\tau^3_{\gamma,\alpha,i} = \sum_{\beta \in B} X_{\alpha,\beta} W^3_{i,\beta} \tau^2_{\gamma,\beta} \quad (3r_T r_V^2 N_o) \quad (2764)$$

$$\tau^4_{\gamma,\alpha} = \sum_{a \in V} W^2_{a,\alpha} Y^3_{a,\gamma} \quad (2r_T r_V N_v) \quad (2765)$$

$$\tau^5_{\gamma,\alpha,i} = \sum_{\delta \in A} Z_{\gamma,\delta} Y^4_{i,\delta} \tau^4_{\delta,\alpha} \quad (3r_T^2 r_V N_o) \quad (2766)$$

$$\tau^6_{\gamma,i,j,k} = \sum_{\alpha \in B} W^1_{i,\alpha} \tau^3_{\gamma,\alpha,j} \tau^5_{\gamma,\alpha,k} \quad (3r_T r_V N_o^3) \quad (2767)$$

$$\tau^7_{i,j,k,l} = \sum_{\gamma \in A} Y^2_{k,\gamma} \tau^6_{\gamma,i,j,l} \quad (2r_T N_o^4) \quad (2768)$$

$$\tau^8_{\gamma,i,j,k} = \sum_{l \in O} Y^4_{l,\gamma} \tau^7_{i,l,j,k} \quad (2r_T N_o^4) \quad (2769)$$

$$\tau^9_{\gamma,\delta,w,i} = \sum_{j \in O} \sum_{k \in O} {}^2D^2_{j,w} {}^2D^4_{k,w} Y^{2,*}_{j,\delta} \tau^1_{\gamma,\delta,w,k} \tau^8_{\gamma,i,k,j} \quad (5r_D r_T^2 N_o^3) \quad (2770)$$

$$\tau^{10}_{\gamma,\delta,w} = \sum_{\epsilon \in A} \sum_{i \in O} Y^2_{i,\gamma} Z_{\gamma,\epsilon} \tau^9_{\epsilon,\delta,w,i} \quad (3r_D r_T^3 N_o) \quad (2771)$$

$${}^{21}R_{a,\gamma} \leftarrow \sum_{\delta \in A} \sum_{w \in D} \frac{1}{4} {}^2D^1_{a,w} Y^1_{a,\delta} \tau^{10}_{\delta,\gamma,w} \quad (3r_D r_T^2 N_v) \quad (2772)$$

Raw expression

$${}^{21}R_{a,\epsilon} \leftarrow \sum_{\gamma \in A} \sum_{i \in O} \sum_{j \in O} \sum_{k \in O} \sum_{l \in O} \sum_{b \in V} \sum_{c \in V} \sum_{d \in V} \frac{1}{4} Y^{2,*}_{i,\epsilon} Z^*_{\epsilon,\gamma} Y^{3,*}_{b,\gamma} Y^{4,*}_{j,\gamma} {}^2D^{a,i,b,j}_{a,\delta} {}^2T_{b,j,a,k} {}^2T_{c,i,d,l} V_{k,d,l,c} \quad (2773)$$

Factorized expression

$$\tau^0_{\gamma,\delta,w} = \sum_{a \in V} {}^2D^3_{a,w} Y^1_{a,\gamma} Y^{3,*}_{a,\delta} \quad (3r_D r_T^2 N_v) \quad (2774)$$

$$\tau^1_{\gamma,\delta,w} = \sum_{i \in O} {}^2D^4_{i,w} Y^2_{i,\gamma} Y^{4,*}_{i,\delta} \quad (3r_D r_T^2 N_o) \quad (2775)$$

$$\tau^2_{\gamma,\delta,w} = \sum_{\epsilon \in A} Z^*_{\delta,\epsilon} \tau^0_{\gamma,\epsilon,w} \tau^1_{\gamma,\epsilon,w} \quad (3r_D r_T^3) \quad (2776)$$

$$\tau^3_{\gamma,\delta,w} = \sum_{\epsilon \in A} Z_{\epsilon,\gamma} \tau^2_{\epsilon,\delta,w} \quad (2r_D r_T^3) \quad (2777)$$

$$\tau^4_{\gamma,\alpha} = \sum_{a \in V} W^2_{a,\alpha} Y^1_{a,\gamma} \quad (2r_T r_V N_v) \quad (2778)$$

$$\tau^5_{\gamma,\alpha,i} = \sum_{\beta \in B} W^1_{i,\beta} X_{\beta,\alpha} \tau^4_{\gamma,\beta} \quad (3r_T r_V^2 N_o) \quad (2779)$$

$$\tau^6_{\gamma,\alpha} = \sum_{i \in O} W^3_{i,\alpha} Y^2_{i,\gamma} \quad (2r_T r_V N_o) \quad (2780)$$

$$\tau^7_{\gamma,\alpha} = \sum_{a \in V} W^4_{a,\alpha} Y^3_{a,\gamma} \quad (2r_T r_V N_v) \quad (2781)$$

$$\tau^8_{\gamma,\delta,i} = \sum_{\alpha \in B} \tau^6_{\gamma,\alpha} \tau^7_{\delta,\alpha} \tau^5_{\gamma,\alpha,i} \quad (3r_T^2 r_V N_o) \quad (2782)$$

$$\tau^9_{\gamma,i} = \sum_{\delta \in A} Z_{\delta,\gamma} \tau^8_{\delta,\gamma,i} \quad (2r_T^2 N_o) \quad (2783)$$

$$\tau^{10}_{i,j} = \sum_{\gamma \in A} Y^4_{j,\gamma} \tau^9_{\gamma,i} \quad (2r_T N_o^2) \quad (2784)$$

$$\tau^{11}_{\gamma,i} = \sum_{j \in O} Y^4_{j,\gamma} \tau^{10}_{j,i} \quad (2r_T N_o^2) \quad (2785)$$

$$\tau^{12}_{\gamma,\delta,w} = \sum_{i \in O} {}^2D^2_{i,w} Y^{2,*}_{i,\delta} \tau^{11}_{\gamma,i} \quad (3r_D r_T^2 N_o) \quad (2786)$$

$${}^{21}R_{a,\gamma} \leftarrow \sum_{\delta \in A} \sum_{w \in D} \frac{1}{4} {}^2D^1_{a,w} Y^3_{a,\delta} \tau^{12}_{\delta,\gamma,w} \tau^3_{\delta,\gamma,w} \quad (4r_D r_T^2 N_v) \quad (2787)$$

Raw expression

$${}^{21}R_{a,\epsilon} \leftarrow \sum_{\gamma \in A} \sum_{i \in O} \sum_{j \in O} \sum_{k \in O} \sum_{l \in O} \sum_{b \in V} \sum_{c \in V} \sum_{d \in V} \frac{1}{4} Y^{2,*}_{i,\epsilon} Z^*_{\epsilon,\gamma} Y^{3,*}_{b,\gamma} Y^{4,*}_{j,\gamma} {}^2D^{a,i,b,j}_{a,\delta} {}^2T_{b,j,a,k} {}^2T_{c,l,d,i} V_{k,c,l,d} \quad (2788)$$

Factorized expression

$$\tau^0_{\gamma,\delta,w} = \sum_{i \in O} {}^2D^2_{i,w} Y^4_{i,\gamma} Y^{2,*}_{i,\delta} \quad (3r_D r_T^2 N_o) \quad (2789)$$

Factorized expression

$$\tau^1_{\gamma,\alpha} = \sum_{a \in V} W^2_{a,\alpha} Y^1_{a,\gamma} \quad (2r_T r_V N_v) \quad (2790)$$

$$\tau^2_{\gamma,\alpha,i} = \sum_{\beta \in B} W^1_{i,\beta} X_{\beta,\alpha} \tau^1_{\gamma,\beta} \quad (3r_T r_V^2 N_o) \quad (2791)$$

$$\tau^3_{\gamma,\alpha} = \sum_{i \in O} W^3_{i,\alpha} Y^2_{i,\gamma} \quad (2r_T r_V N_o) \quad (2792)$$

$$\tau^4_{\gamma,\alpha} = \sum_{a \in V} W^4_{a,\alpha} Y^3_{a,\gamma} \quad (2r_T r_V N_v) \quad (2793)$$

$$\tau^5_{\gamma,\delta,i} = \sum_{\alpha \in B} \tau^3_{\gamma,\alpha} \tau^4_{\delta,\alpha} \tau^2_{\gamma,\alpha,i} \quad (3r_T^2 r_V N_o) \quad (2794)$$

$$\tau^6_{\gamma,i} = \sum_{\delta \in A} Z_{\delta,\gamma} \tau^5_{\delta,\gamma,i} \quad (2r_T^2 N_o) \quad (2795)$$

$$\tau^7_{i,j} = \sum_{\gamma \in A} Y^4_{j,\gamma} \tau^6_{\gamma,i} \quad (2r_T N_o^2) \quad (2796)$$

$$\tau^8_{\gamma,i} = \sum_{j \in O} Y^2_{j,\gamma} \tau^7_{j,i} \quad (2r_T N_o^2) \quad (2797)$$

$$\tau^9_{\gamma,\delta,w} = \sum_{i \in O} {}^2D^4_{i,w} Y^{4,*}_{i,\delta} \tau^8_{\gamma,i} \quad (3r_D r_T^2 N_o) \quad (2798)$$

$$\tau^{10}_{\gamma,\delta,w} = \sum_{a \in V} {}^2D^3_{a,w} Y^1_{a,\gamma} Y^{3,*}_{a,\delta} \quad (3r_D r_T^2 N_v) \quad (2799)$$

$$\tau^{11}_{\gamma,\delta,w} = \sum_{\epsilon \in A} Z^*_{\delta,\epsilon} \tau^{10}_{\gamma,\epsilon,w} \tau^9_{\gamma,\epsilon,w} \quad (3r_D r_T^3) \quad (2800)$$

$$\tau^{12}_{\gamma,\delta,w} = \sum_{\epsilon \in A} Z_{\epsilon,\gamma} \tau^{11}_{\epsilon,\delta,w} \quad (2r_D r_T^3) \quad (2801)$$

$${}^{21}R_{a,\gamma} \leftarrow \sum_{\delta \in A} \sum_{w \in D} \frac{1}{4} {}^2D^1_{a,w} Y^3_{a,\delta} \tau^0_{\delta,\gamma,w} \tau^{12}_{\delta,\gamma,w} \quad (4r_D r_T^2 N_v) \quad (2802)$$

Raw expression

$${}^{21}R_{a,\epsilon} \leftarrow \sum_{\gamma \in A} \sum_{i \in O} \sum_{j \in O} \sum_{k \in O} \sum_{l \in O} \sum_{b \in V} \sum_{c \in V} \sum_{d \in V} \frac{1}{4} Y^{2,*}_{i,\epsilon} Z^*_{\epsilon,\gamma} Y^{3,*}_{b,\gamma} Y^{4,*}_{j,\gamma} {}^2D^{a,i,b,j}_{c,k,a,l} {}^2T_{b,j,d,i} {}^2T_{c,k,a,l} V_{k,d,l,c} \quad (2803)$$

$$\tau^0_{\gamma,\alpha} = \sum_{a \in V} W^2_{a,\alpha} Y^3_{a,\gamma} \quad (2r_T r_V N_v) \quad (2804)$$

$$\tau^1_{\gamma,\alpha,i} = \sum_{\beta \in B} W^1_{i,\beta} X_{\beta,\alpha} \tau^0_{\gamma,\beta} \quad (3r_T r_V^2 N_o) \quad (2805)$$

$$\tau^2_{\gamma,\alpha} = \sum_{i \in O} W^3_{i,\alpha} Y^4_{i,\gamma} \quad (2r_T r_V N_o) \quad (2806)$$

$$\tau^3_{\gamma,\alpha} = \sum_{a \in V} W^4_{a,\alpha} Y^1_{a,\gamma} \quad (2r_T r_V N_v) \quad (2807)$$

$$\tau^4_{\gamma,\delta,i} = \sum_{\alpha \in B} \tau^2_{\delta,\alpha} \tau^3_{\gamma,\alpha} \tau^1_{\delta,\alpha,i} \quad (3r_T^2 r_V N_o) \quad (2808)$$

$$\tau^5_{\gamma,i} = \sum_{\delta \in A} Z_{\gamma,\delta} \tau^4_{\gamma,\delta,i} \quad (2r_T^2 N_o) \quad (2809)$$

$$\tau^6_{i,j} = \sum_{\gamma \in A} Y^2_{j,\gamma} \tau^5_{\gamma,i} \quad (2r_T N_o^2) \quad (2810)$$

$$\tau^7_{\gamma,i} = \sum_{j \in O} Y^4_{j,\gamma} \tau^6_{j,i} \quad (2r_T N_o^2) \quad (2811)$$

$$\tau^8_{\gamma,\delta,w} = \sum_{i \in O} {}^2D^2_{i,w} Y^{2,*}_{i,\delta} \tau^7_{\gamma,i} \quad (3r_D r_T^2 N_o) \quad (2812)$$

$$\tau^9_{\gamma,\delta,w} = \sum_{a \in V} {}^2D^3_{a,w} Y^1_{a,\gamma} Y^{3,*}_{a,\delta} \quad (3r_D r_T^2 N_v) \quad (2813)$$

$$\tau^{10}_{\gamma,\delta,w} = \sum_{i \in O} {}^2D^4_{i,w} Y^2_{i,\gamma} Y^{4,*}_{i,\delta} \quad (3r_D r_T^2 N_o) \quad (2814)$$

$$\tau^{11}_{\gamma,\delta,w} = \sum_{\epsilon \in A} Z^*_{\delta,\epsilon} \tau^{10}_{\gamma,\epsilon,w} \tau^9_{\gamma,\epsilon,w} \quad (3r_D r_T^3) \quad (2815)$$

$$\tau^{12}_{\gamma,\delta,w} = \sum_{\epsilon \in A} Z_{\epsilon,\gamma} \tau^{11}_{\epsilon,\delta,w} \quad (2r_D r_T^3) \quad (2816)$$

$${}^{21}R_{a,\gamma} \leftarrow \sum_{\delta \in A} \sum_{w \in D} \frac{1}{4} {}^2D^1_{a,w} Y^3_{a,\delta} \tau^{12}_{\delta,\gamma,w} \tau^8_{\delta,\gamma,w} \quad (4r_D r_T^2 N_v) \quad (2817)$$

Raw expression

$${}^{21}R_{a,\epsilon} \leftarrow \sum_{\gamma \in A} \sum_{i \in O} \sum_{j \in O} \sum_{k \in O} \sum_{l \in O} \sum_{b \in V} \sum_{c \in V} \sum_{d \in V} \frac{1}{4} Y^{2,*}_{i,\epsilon} Z^*_{\epsilon,\gamma} Y^{3,*}_{b,\gamma} Y^{4,*}_{j,\gamma} {}^2D^{a,i,b,j} {}^2T_{b,j,d,l} {}^2T_{c,i,a,k} V_{k,d,l,c} \quad (2818)$$

Factorized expression

$$\tau^0_{\gamma,\delta,w} = \sum_{a \in V} {}^2D^3_{a,w} Y^1_{a,\gamma} Y^{3,*}_{a,\delta} (3r_D r_T^2 N_v) \quad (2819)$$

$$\tau^1_{\gamma,\delta,w} = \sum_{i \in O} {}^2D^4_{i,w} Y^2_{i,\gamma} Y^{4,*}_{i,\delta} (3r_D r_T^2 N_o) \quad (2820)$$

$$\tau^2_{\gamma,\delta,w} = \sum_{\epsilon \in A} Z^*_{\delta,\epsilon} \tau^0_{\gamma,\epsilon,w} \tau^1_{\gamma,\epsilon,w} (3r_D r_T^3) \quad (2821)$$

$$\tau^3_{\gamma,\delta,w} = \sum_{\epsilon \in A} Z_{\epsilon,\gamma} \tau^2_{\epsilon,\delta,w} (2r_D r_T^3) \quad (2822)$$

$$\tau^4_{\gamma,\delta,w} = \sum_{i \in O} {}^2D^2_{i,w} Y^4_{i,\gamma} Y^{2,*}_{i,\delta} (3r_D r_T^2 N_o) \quad (2823)$$

$$\tau^5_{\gamma,\alpha} = \sum_{a \in V} W^4_{a,\alpha} Y^1_{a,\gamma} (2r_T r_V N_v) \quad (2824)$$

$$\tau^6_{\gamma,\alpha,i} = \sum_{\beta \in B} X_{\alpha,\beta} W^3_{i,\beta} \tau^5_{\gamma,\beta} (3r_T r_V^2 N_o) \quad (2825)$$

$$\tau^7_{\gamma,\alpha} = \sum_{i \in O} W^1_{i,\alpha} Y^2_{i,\gamma} (2r_T r_V N_o) \quad (2826)$$

$$\tau^8_{\gamma,\alpha} = \sum_{\delta \in A} \sum_{i \in O} Z_{\delta,\gamma} Y^4_{i,\gamma} \tau^7_{\delta,\alpha} \tau^6_{\delta,\alpha,i} (4r_T^2 r_V N_o) \quad (2827)$$

$$\tau^9_{\gamma,a} = \sum_{\alpha \in B} W^2_{a,\alpha} \tau^8_{\gamma,\alpha} (2r_T r_V N_v) \quad (2828)$$

$$\tau^{10}_{a,b} = \sum_{\gamma \in A} Y^3_{b,\gamma} \tau^9_{\gamma,a} (2r_T N_v^2) \quad (2829)$$

$$\tau^{11}_{\gamma,a} = \sum_{b \in V} Y^3_{b,\gamma} \tau^{10}_{b,a} (2r_T N_v^2) \quad (2830)$$

$${}^{21}R_{a,\gamma} \leftarrow \sum_{\delta \in A} \sum_{w \in D} \frac{1}{4} {}^2D^1_{a,w} \tau^{11}_{\delta,a} \tau^3_{\delta,\gamma,w} \tau^4_{\delta,\gamma,w} (4r_D r_T^2 N_v) \quad (2831)$$

Raw expression

$${}^{21}R_{a,\epsilon} \leftarrow \sum_{\gamma \in A} \sum_{i \in O} \sum_{j \in O} \sum_{k \in O} \sum_{l \in O} \sum_{b \in V} \sum_{c \in V} \sum_{d \in V} \frac{1}{4} Y^{2,*}_{i,\epsilon} Z^*_{\epsilon,\gamma} Y^{3,*}_{b,\gamma} Y^{4,*}_{j,\gamma} {}^2D^{a,i,b,j} {}^2T_{b,k,a,i} {}^2T_{c,j,d,l} V_{k,d,l,c} \quad (2832)$$

Factorized expression

$$\tau^0_{\gamma,\alpha} = \sum_{a \in V} W^2_{a,\alpha} Y^1_{a,\gamma} (2r_T r_V N_v) \quad (2833)$$

$$\tau^1_{\gamma,\alpha,i} = \sum_{\delta \in A} Y^2_{i,\delta} Z_{\delta,\gamma} \tau^0_{\delta,\alpha} (3r_T^2 r_V N_o) \quad (2834)$$

$$\tau^2_{\gamma,\alpha} = \sum_{i \in O} W^1_{i,\alpha} Y^4_{i,\gamma} (2r_T r_V N_o) \quad (2835)$$

$$\tau^3_{\gamma,\delta,w} = \sum_{a \in V} {}^2D^3_{a,w} Y^1_{a,\gamma} Y^{3,*}_{a,\delta} (3r_D r_T^2 N_v) \quad (2836)$$

$$\tau^4_{\gamma,\alpha} = \sum_{i \in O} W^3_{i,\alpha} Y^2_{i,\gamma} (2r_T r_V N_o) \quad (2837)$$

$$\tau^5_{\gamma,\alpha} = \sum_{a \in V} W^4_{a,\alpha} Y^3_{a,\gamma} (2r_T r_V N_v) \quad (2838)$$

$$\tau^6_{\gamma,\alpha,i} = \sum_{\delta \in A} Z_{\gamma,\delta} Y^4_{i,\delta} \tau^5_{\delta,\alpha} (3r_T^2 r_V N_o) \quad (2839)$$

$$\tau^7_{\gamma,\alpha,w} = \sum_{\delta \in A} \sum_{i \in O} {}^2D^4_{i,w} Y^{4,*}_{i,\gamma} \tau^4_{\delta,\alpha} \tau^3_{\delta,\gamma,w} \tau^6_{\delta,\alpha,i} (5r_D r_T^2 r_V N_o) \quad (2840)$$

$$\tau^8_{\gamma,\alpha,w} = \sum_{\beta \in B} X_{\alpha,\beta} \tau^7_{\gamma,\beta,w} (2r_D r_T r_V^2) \quad (2841)$$

$$\tau^9_{\gamma,\alpha,w} = \sum_{\delta \in A} Z^*_{\gamma,\delta} \tau^8_{\delta,\alpha,w} (2r_D r_T^2 r_V) \quad (2842)$$

$$\tau^{10}_{\gamma,\delta,w,i} = \sum_{\alpha \in B} \tau^2_{\gamma,\alpha} \tau^1_{\gamma,\alpha,i} \tau^9_{\delta,\alpha,w} (3r_D r_T^2 r_V N_o) \quad (2843)$$

$$\tau^{11}_{\gamma,\delta,w} = \sum_{i \in O} {}^2D^2_{i,w} Y^{2,*}_{i,\delta} \tau^{10}_{\gamma,\delta,w,i} (3r_D r_T^2 N_o) \quad (2844)$$



$${}^{21}R_{a,\gamma} \leftarrow \sum_{\delta \in A} \sum_{w \in D} \frac{1}{4} {}^2D^1_{a,w} Y^3_{a,\delta} \tau^{11}_{\delta,\gamma,w} \quad (3r_D r_T^2 N_v) \quad (2845)$$

Raw expression

$${}^{21}R_{a,\epsilon} \leftarrow \sum_{\gamma \in A} \sum_{i \in O} \sum_{j \in O} \sum_{k \in O} \sum_{l \in O} \sum_{b \in V} \sum_{c \in V} \sum_{d \in V} \frac{1}{4} Y^{2,*}_{i,\epsilon} Z^*_{\epsilon,\gamma} Y^{3,*}_{b,\gamma} Y^{4,*}_{j,\gamma} {}^2D^{a,i,b,j} {}^2T_{b,k,a,i} {}^2T_{c,l,d,j} V_{k,c,l,d} \quad (2846)$$

Factorized expression

$$\tau^0_{\gamma,\delta,w} = \sum_{a \in V} {}^2D^3_{a,w} Y^1_{a,\gamma} Y^{3,*}_{a,\delta} \quad (3r_D r_T^2 N_v) \quad (2847)$$

$$\tau^1_{\gamma,\delta,w,i} = \sum_{\epsilon \in A} Z^*_{\delta,\epsilon} Y^{4,*}_{i,\epsilon} \tau^0_{\gamma,\epsilon,w} \quad (3r_D r_T^3 N_o) \quad (2848)$$

$$\tau^2_{\gamma,\alpha} = \sum_{a \in V} W^2_{a,\alpha} Y^1_{a,\gamma} \quad (2r_T r_V N_v) \quad (2849)$$

$$\tau^3_{\gamma,\alpha,i} = \sum_{\beta \in B} W^1_{i,\beta} X_{\beta,\alpha} \tau^2_{\gamma,\beta} \quad (3r_T r_V^2 N_o) \quad (2850)$$

$$\tau^4_{\gamma,\alpha} = \sum_{a \in V} W^4_{a,\alpha} Y^3_{a,\gamma} \quad (2r_T r_V N_v) \quad (2851)$$

$$\tau^5_{\gamma,\alpha,i} = \sum_{\delta \in A} Z_{\gamma,\delta} Y^4_{i,\delta} \tau^4_{\delta,\alpha} \quad (3r_T^2 r_V N_o) \quad (2852)$$

$$\tau^6_{\gamma,i,j,k} = \sum_{\alpha \in B} W^3_{j,\alpha} \tau^3_{\gamma,\alpha,i} \tau^5_{\gamma,\alpha,k} \quad (3r_T r_V N_o^3) \quad (2853)$$

$$\tau^7_{i,j,k,l} = \sum_{\gamma \in A} Y^2_{k,\gamma} \tau^6_{\gamma,i,j,l} \quad (2r_T N_o^4) \quad (2854)$$

$$\tau^8_{\gamma,i,j,k} = \sum_{l \in O} Y^2_{l,\gamma} \tau^7_{l,i,j,k} \quad (2r_T N_o^4) \quad (2855)$$

$$\tau^9_{\gamma,\delta,w,i} = \sum_{j \in O} \sum_{k \in O} {}^2D^2_{j,w} {}^2D^4_{k,w} Y^{2,*}_{j,\delta} \tau^1_{\gamma,\delta,w,k} \tau^8_{\gamma,i,k,j} \quad (5r_D r_T^2 N_o^3) \quad (2856)$$

$$\tau^{10}_{\gamma,\delta,w} = \sum_{\epsilon \in A} \sum_{i \in O} Z_{\epsilon,\gamma} Y^4_{i,\gamma} \tau^9_{\epsilon,\delta,w,i} \quad (3r_D r_T^3 N_o) \quad (2857)$$

$${}^{21}R_{a,\gamma} \leftarrow \sum_{\delta \in A} \sum_{w \in D} \frac{1}{4} {}^2D^1_{a,w} Y^3_{a,\delta} \tau^{10}_{\delta,\gamma,w} \quad (3r_D r_T^2 N_v) \quad (2858)$$

Raw expression

$${}^{21}R_{a,\epsilon} \leftarrow \sum_{\gamma \in A} \sum_{i \in O} \sum_{j \in O} \sum_{k \in O} \sum_{l \in O} \sum_{b \in V} \sum_{c \in V} \sum_{d \in V} \frac{1}{4} Y^{2,*}_{i,\epsilon} Z^*_{\epsilon,\gamma} Y^{3,*}_{b,\gamma} Y^{4,*}_{j,\gamma} {}^2D^{a,i,b,j} {}^2T_{b,k,a,l} {}^2T_{c,i,d,j} V_{k,d,l,c} \quad (2859)$$

Factorized expression

$$\tau^0_{\gamma,\delta,w} = \sum_{a \in V} {}^2D^3_{a,w} Y^1_{a,\gamma} Y^{3,*}_{a,\delta} \quad (3r_D r_T^2 N_v) \quad (2860)$$

$$\tau^1_{\gamma,\delta,w} = \sum_{i \in O} {}^2D^4_{i,w} Y^2_{i,\gamma} Y^{4,*}_{i,\delta} \quad (3r_D r_T^2 N_o) \quad (2861)$$

$$\tau^2_{\gamma,\delta,w} = \sum_{\epsilon \in A} Z^*_{\delta,\epsilon} \tau^0_{\gamma,\epsilon,w} \tau^1_{\gamma,\epsilon,w} \quad (3r_D r_T^3) \quad (2862)$$

$$\tau^3_{\gamma,\delta,w} = \sum_{\epsilon \in A} Z_{\epsilon,\gamma} \tau^2_{\epsilon,\delta,w} \quad (2r_D r_T^3) \quad (2863)$$

$$\tau^4_{\gamma,\alpha} = \sum_{a \in V} W^2_{a,\alpha} Y^3_{a,\gamma} \quad (2r_T r_V N_v) \quad (2864)$$

$$\tau^5_{\gamma,\alpha,i} = \sum_{\beta \in B} W^1_{i,\beta} X_{\beta,\alpha} \tau^4_{\gamma,\beta} \quad (3r_T r_V^2 N_o) \quad (2865)$$

$$\tau^6_{\gamma,\alpha} = \sum_{i \in O} W^3_{i,\alpha} Y^4_{i,\gamma} \quad (2r_T r_V N_o) \quad (2866)$$

$$\tau^7_{\gamma,\alpha} = \sum_{a \in V} W^4_{a,\alpha} Y^1_{a,\gamma} \quad (2r_T r_V N_v) \quad (2867)$$

$$\tau^8_{\gamma,\delta,i} = \sum_{\alpha \in B} \tau^6_{\delta,\alpha} \tau^7_{\gamma,\alpha} \tau^5_{\delta,\alpha,i} \quad (3r_T^2 r_V N_o) \quad (2868)$$

$$\tau^9_{\gamma,\delta,\epsilon} = \sum_{i \in O} Z_{\gamma,\delta} Y^4_{i,\delta} \tau^8_{\gamma,\epsilon,i} \quad (3r_T^3 N_o) \quad (2869)$$

$$\tau^{10}_{\gamma,\delta,i} = \sum_{\epsilon \in A} Y^2_{i,\epsilon} \tau^9_{\epsilon,\gamma,\delta} \quad (2r_T^3 N_o) \quad (2870)$$

$$\tau^{11}_{\gamma,\delta,w} = \sum_{\epsilon \in A} \sum_{i \in O} {}^2D^2_{i,w} Y^{2,*}_{i,\delta} \tau^{10}_{\gamma,\epsilon,i} \tau^3_{\epsilon,\delta,w} \quad (4r_D r_T^3 N_o) \quad (2871)$$

$$\tau^{10}_{\gamma,\delta,w} = \sum_{\epsilon \in A} \sum_{i \in O} Z_{\epsilon,\gamma} Y^4_{i,\gamma} \tau^9_{\epsilon,\delta,w,i} \quad (3r_D r_T^3 N_o) \quad (2884)$$

$${}^{21}R_{a,\gamma} \leftarrow \sum_{\delta \in A} \sum_{w \in D} \frac{1}{4} {}^2D^1_{a,w} Y^3_{a,\delta} \tau^{11}_{\delta,\gamma,w} \quad (3r_D r_T^2 N_v) \quad (2872)$$

$${}^{21}R_{a,\gamma} \leftarrow \sum_{\delta \in A} \sum_{w \in D} \frac{1}{4} {}^2D^1_{a,w} Y^3_{a,\delta} \tau^{10}_{\delta,\gamma,w} \quad (3r_D r_T^2 N_v) \quad (2885)$$

Raw expression

$${}^{21}R_{a,\epsilon} \leftarrow \sum_{\gamma \in A} \sum_{i \in O} \sum_{j \in O} \sum_{k \in O} \sum_{l \in O} \sum_{b \in V} \sum_{c \in V} \sum_{d \in V} \frac{1}{4} Y^{2,*}_{i,\epsilon} Z^*_{\epsilon,\gamma} Y^{3,*}_{b,\gamma} Y^{4,*}_{j,\gamma} {}^2D^{a,i,b,j} {}^2T_{b,k,a,l} {}^2T_{c,j,d,i} V_{k,c,l,d} \quad (2873)$$

Raw expression

$${}^{21}R_{a,\epsilon} \leftarrow \sum_{\gamma \in A} \sum_{i \in O} \sum_{j \in O} \sum_{k \in O} \sum_{l \in O} \sum_{b \in V} \sum_{c \in V} \sum_{d \in V} \frac{1}{4} Y^{2,*}_{i,\epsilon} Z^*_{\epsilon,\gamma} Y^{3,*}_{b,\gamma} Y^{4,*}_{j,\gamma} {}^2D^{a,i,b,j} {}^2T_{b,k,d,l} {}^2T_{c,j,a,i} V_{k,d,l,c} \quad (2886)$$

Factorized expression

$$\tau^0_{\gamma,\delta,w} = \sum_{a \in V} {}^2D^3_{a,w} Y^1_{a,\gamma} Y^{3,*}_{a,\delta} \quad (3r_D r_T^2 N_v) \quad (2874)$$

$$\tau^0_{\gamma,\delta,w} = \sum_{i \in O} {}^2D^2_{i,w} Y^4_{i,\gamma} Y^{2,*}_{i,\delta} \quad (3r_D r_T^2 N_o) \quad (2887)$$

$$\tau^1_{\gamma,\delta,w,i} = \sum_{\epsilon \in A} Z^*_{\delta,\epsilon} Y^{4,*}_{i,\epsilon} \tau^0_{\gamma,\epsilon,w} \quad (3r_D r_T^3 N_o) \quad (2875)$$

$$\tau^1_{\gamma,\alpha} = \sum_{a \in V} W^2_{a,\alpha} Y^3_{a,\gamma} \quad (2r_T r_V N_v) \quad (2888)$$

$$\tau^2_{\gamma,\alpha} = \sum_{a \in V} W^4_{a,\alpha} Y^1_{a,\gamma} \quad (2r_T r_V N_v) \quad (2876)$$

$$\tau^2_{\gamma,\alpha,i} = \sum_{\beta \in B} W^1_{i,\beta} X_{\beta,\alpha} \tau^1_{\gamma,\beta} \quad (3r_T r_V^2 N_o) \quad (2889)$$

$$\tau^3_{\gamma,\alpha,i} = \sum_{\beta \in B} X_{\alpha,\beta} W^3_{i,\beta} \tau^2_{\gamma,\beta} \quad (3r_T r_V^2 N_o) \quad (2877)$$

$$\tau^3_{\gamma,\alpha} = \sum_{i \in O} W^3_{i,\alpha} Y^4_{i,\gamma} \quad (2r_T r_V N_o) \quad (2890)$$

$$\tau^4_{\gamma,\alpha} = \sum_{a \in V} W^2_{a,\alpha} Y^3_{a,\gamma} \quad (2r_T r_V N_v) \quad (2878)$$

$$\tau^4_{\gamma,\alpha} = \sum_{a \in V} W^4_{a,\alpha} Y^1_{a,\gamma} \quad (2r_T r_V N_v) \quad (2891)$$

$$\tau^5_{\gamma,\alpha,i} = \sum_{\delta \in A} Z_{\gamma,\delta} Y^4_{i,\delta} \tau^4_{\delta,\alpha} \quad (3r_T^2 r_V N_o) \quad (2879)$$

$$\tau^5_{\gamma,\delta,i} = \sum_{\alpha \in B} \tau^3_{\delta,\alpha} \tau^4_{\gamma,\alpha} \tau^2_{\delta,\alpha,i} \quad (3r_T^2 r_V N_o) \quad (2892)$$

$$\tau^6_{\gamma,i,j,k} = \sum_{\alpha \in B} W^1_{i,\alpha} \tau^3_{\gamma,\alpha,j} \tau^5_{\gamma,\alpha,k} \quad (3r_T r_V N_o^3) \quad (2880)$$

$$\tau^6_{\gamma,i} = \sum_{\delta \in A} Z_{\gamma,\delta} \tau^5_{\gamma,\delta,i} \quad (2r_T^2 N_o) \quad (2893)$$

$$\tau^7_{i,j,k,l} = \sum_{\gamma \in A} Y^2_{k,\gamma} \tau^6_{\gamma,i,j,l} \quad (2r_T N_o^4) \quad (2881)$$

$$\tau^7_{i,j} = \sum_{\gamma \in A} Y^2_{j,\gamma} \tau^6_{\gamma,i} \quad (2r_T N_o^2) \quad (2894)$$

$$\tau^8_{\gamma,i,j,k} = \sum_{l \in O} Y^2_{l,\gamma} \tau^7_{l,i,j,k} \quad (2r_T N_o^4) \quad (2882)$$

$$\tau^8_{\gamma,i} = \sum_{j \in O} Y^2_{j,\gamma} \tau^7_{j,i} \quad (2r_T N_o^2) \quad (2895)$$

$$\tau^9_{\gamma,\delta,w,i} = \sum_{j \in O} \sum_{k \in O} {}^2D^2_{j,w} {}^2D^4_{k,w} Y^{2,*}_{j,\delta} \tau^1_{\gamma,\delta,w,k} \tau^8_{\gamma,i,j,k} \quad (5r_D r_T^2 N_o^3) \quad (2883)$$

$$\tau^9_{\gamma,\delta,w} = \sum_{i \in O} {}^2D^4_{i,w} Y^{4,*}_{i,\delta} \tau^8_{\gamma,i} \quad (3r_D r_T^2 N_o) \quad (2896)$$

$$\tau^{10}_{\gamma,\delta,w} = \sum_{a \in V} {}^2D^3_{a,w} Y^1_{a,\gamma} Y^{3,*}_{a,\delta} \quad (3r_D r_T^2 N_v) \quad (2897)$$

$$\tau^8_{\gamma,a} = \sum_{\delta \in A} Y^1_{a,\delta} \tau^7_{\gamma,\delta} \quad (2r_T^2 N_v) \quad (2910)$$

$$\tau^{11}_{\gamma,\delta,w} = \sum_{\epsilon \in A} Z^*_{\delta,\epsilon} \tau^{10}_{\gamma,\epsilon,w} \tau^9_{\gamma,\epsilon,w} \quad (3r_D r_T^3) \quad (2898)$$

$$\tau^9_{\gamma,\delta,w} = \sum_{a \in V} {}^2D^3_{a,w} Y^{3,*}_{a,\delta} \tau^8_{\gamma,a} \quad (3r_D r_T^2 N_v) \quad (2911)$$

$$\tau^{12}_{\gamma,\delta,w} = \sum_{\epsilon \in A} Z_{\epsilon,\gamma} \tau^{11}_{\epsilon,\delta,w} \quad (2r_D r_T^3) \quad (2899)$$

$$\tau^{10}_{\gamma,\delta,w} = \sum_{\epsilon \in A} Z^*_{\delta,\epsilon} \tau^1_{\gamma,\epsilon,w} \tau^9_{\gamma,\epsilon,w} \quad (3r_D r_T^3) \quad (2912)$$

$${}^{21}R_{a,\gamma} \leftarrow \sum_{\delta \in A} \sum_{w \in D} \frac{1}{4} {}^2D^1_{a,w} Y^3_{a,\delta} \tau^0_{\delta,\gamma,w} \tau^{12}_{\delta,\gamma,w} \quad (4r_D r_T^2 N_v) \quad (2900)$$

$$\tau^{11}_{\gamma,\delta,w} = \sum_{\epsilon \in A} Z_{\epsilon,\gamma} \tau^{10}_{\epsilon,\delta,w} \quad (2r_D r_T^3) \quad (2913)$$

Raw expression

$${}^{21}R_{a,\epsilon} \leftarrow \sum_{\gamma \in A} \sum_{i \in O} \sum_{j \in O} \sum_{k \in O} \sum_{l \in O} \sum_{b \in V} \sum_{c \in V} \sum_{d \in V} \frac{1}{4} Y^{2,*}_{i,\epsilon} Z^*_{\epsilon,\gamma} Y^{3,*}_{b,\gamma} Y^{4,*}_{j,\gamma} {}^2D^{a,i,b,j} {}^2T_{b,l,d,i} {}^2T_{c,j,a,k} V_{k,d,l,c} \quad (2901)$$

$${}^{21}R_{a,\gamma} \leftarrow \sum_{\delta \in A} \sum_{w \in D} \frac{1}{4} {}^2D^1_{a,w} Y^3_{a,\delta} \tau^0_{\delta,\gamma,w} \tau^{11}_{\delta,\gamma,w} \quad (4r_D r_T^2 N_v) \quad (2914)$$

Raw expression

$${}^{21}R_{a,\epsilon} \leftarrow \sum_{\gamma \in A} \sum_{i \in O} \sum_{j \in O} \sum_{k \in O} \sum_{l \in O} \sum_{b \in V} \sum_{c \in V} \sum_{d \in V} \frac{1}{4} Y^{2,*}_{i,\epsilon} Z^*_{\epsilon,\gamma} Y^{3,*}_{b,\gamma} Y^{4,*}_{j,\gamma} {}^2D^{a,i,b,j} {}^2T_{b,l,d,j} {}^2T_{c,i,a,k} V_{k,c,l,d} \quad (2915)$$

Factorized expression

$$\tau^0_{\gamma,\delta,w} = \sum_{i \in O} {}^2D^2_{i,w} Y^4_{i,\gamma} Y^{2,*}_{i,\delta} \quad (3r_D r_T^2 N_o) \quad (2902)$$

Factorized expression

$$\tau^1_{\gamma,\delta,w} = \sum_{i \in O} {}^2D^4_{i,w} Y^2_{i,\gamma} Y^{4,*}_{i,\delta} \quad (3r_D r_T^2 N_o) \quad (2903)$$

$$\tau^0_{\gamma,\alpha} = \sum_{a \in V} W^2_{a,\alpha} Y^3_{a,\gamma} \quad (2r_T r_V N_v) \quad (2916)$$

$$\tau^2_{\gamma,\alpha} = \sum_{a \in V} W^2_{a,\alpha} Y^3_{a,\gamma} \quad (2r_T r_V N_v) \quad (2904)$$

$$\tau^1_{\gamma,\alpha,i} = \sum_{\beta \in B} W^1_{i,\beta} X_{\beta,\alpha} \tau^0_{\gamma,\beta} \quad (3r_T r_V^2 N_o) \quad (2917)$$

$$\tau^3_{\gamma,\alpha,i} = \sum_{\beta \in B} W^1_{i,\beta} X_{\beta,\alpha} \tau^2_{\gamma,\beta} \quad (3r_T r_V^2 N_o) \quad (2905)$$

$$\tau^2_{\gamma,\delta,\alpha} = \sum_{i \in O} Y^4_{i,\delta} \tau^1_{\gamma,\alpha,i} \quad (2r_T^2 r_V N_o) \quad (2918)$$

$$\tau^4_{\gamma,\alpha} = \sum_{i \in O} W^3_{i,\alpha} Y^4_{i,\gamma} \quad (2r_T r_V N_o) \quad (2906)$$

$$\tau^3_{\gamma,\alpha} = \sum_{a \in V} W^4_{a,\alpha} Y^1_{a,\gamma} \quad (2r_T r_V N_v) \quad (2919)$$

$$\tau^5_{\gamma,\alpha} = \sum_{\delta \in A} \sum_{i \in O} Y^2_{i,\gamma} Z_{\gamma,\delta} \tau^4_{\delta,\alpha} \tau^3_{\delta,\alpha,i} \quad (4r_T^2 r_V N_o) \quad (2907)$$

$$\tau^4_{\gamma,\alpha,i} = \sum_{\delta \in A} Y^2_{i,\delta} Z_{\delta,\gamma} \tau^3_{\delta,\alpha} \quad (3r_T^2 r_V N_o) \quad (2920)$$

$$\tau^6_{\gamma,a} = \sum_{\alpha \in B} W^4_{a,\alpha} \tau^5_{\gamma,\alpha} \quad (2r_T r_V N_v) \quad (2908)$$

$$\tau^5_{\gamma,\delta,\alpha,w} = \sum_{i \in O} {}^2D^4_{i,w} Y^{4,*}_{i,\delta} \tau^4_{\gamma,\alpha,i} \quad (3r_D r_T^2 r_V N_o) \quad (2921)$$

$$\tau^7_{\gamma,\delta} = \sum_{a \in V} Y^1_{a,\gamma} \tau^6_{\delta,a} \quad (2r_T^2 N_v) \quad (2909)$$

$$\tau^6_{\gamma,\delta,w} = \sum_{a \in V} {}^2D^3_{a,w} Y^1_{a,\gamma} Y^{3,*}_{a,\delta} \quad (3r_D r_T^2 N_v) \quad (2922)$$

$$\tau_{\gamma,\delta,w,i}^7 = \sum_{\epsilon \in A} Y_{i,\epsilon}^2 Z_{\epsilon,\gamma} \tau_{\epsilon,\delta,w}^6 \quad (3r_D r_T^3 N_o) \quad (2923)$$

$$\tau_{\gamma,\alpha}^5 = \sum_{a \in V} W_{a,\alpha}^2 Y_{a,\gamma}^3 \quad (2r_T r_V N_v) \quad (2935)$$

$$\tau_{\gamma,\delta,\alpha,w}^8 = \sum_{i \in O} W_{i,\alpha}^3 \tau_{\gamma,\delta,w,i}^7 \quad (2r_D r_T^2 r_V N_o) \quad (2924)$$

$$\tau_{\gamma,\delta,i}^6 = \sum_{\alpha \in B} \tau_{\gamma,\alpha}^4 \tau_{\delta,\alpha}^5 \tau_{\gamma,\alpha,i}^3 \quad (3r_T^2 r_V N_o) \quad (2936)$$

$$\tau_{\gamma,\delta,\epsilon,w}^9 = \sum_{\alpha \in B} \tau_{\gamma,\delta,\alpha}^2 \tau_{\delta,\epsilon,\alpha,w}^5 \tau_{\gamma,\epsilon,\alpha,w}^8 \quad (3r_D r_T^3 r_V) \quad (2925)$$

$$\tau_{\gamma,\delta,\epsilon}^7 = \sum_{i \in O} Y_{i,\delta}^2 Z_{\delta,\epsilon} \tau_{\gamma,\epsilon,i}^6 \quad (3r_T^3 N_o) \quad (2937)$$

$$\tau_{\gamma,\delta,i}^8 = \sum_{\epsilon \in A} Y_{i,\epsilon}^4 \tau_{\gamma,\delta,\epsilon}^7 \quad (2r_T^3 N_o) \quad (2938)$$

$$\tau_{\gamma,\delta,w,i}^{10} = \sum_{\epsilon \in A} {}^2D_{i,w}^2 Y_{i,\epsilon}^4 \tau_{\epsilon,\gamma,\delta,w}^9 \quad (3r_D r_T^3 N_o) \quad (2926)$$

$$\tau_{\gamma,\delta,w}^9 = \sum_{\epsilon \in A} \sum_{i \in O} {}^2D_{i,w}^4 Y_{i,\delta}^{4,*} \tau_{\epsilon,\delta,w}^1 \tau_{\gamma,\epsilon,i}^8 \quad (4r_D r_T^3 N_o) \quad (2939)$$

$$\tau_{\gamma,\delta,w}^{11} = \sum_{\epsilon \in A} \sum_{i \in O} Y_{i,\delta}^{2,*} Z_{\delta,\epsilon}^* \tau_{\gamma,\epsilon,w,i}^{10} \quad (3r_D r_T^3 N_o) \quad (2927)$$

$$\tau_{\gamma,\delta,w}^{10} = \sum_{\epsilon \in A} Z_{\delta,\epsilon}^* \tau_{\gamma,\epsilon,w}^9 \quad (2r_D r_T^3) \quad (2940)$$

$${}^{21}R_{a,\gamma} \leftarrow \sum_{\delta \in A} \sum_{w \in D} \frac{1}{4} {}^2D_{a,w}^1 Y_{a,\delta}^3 \tau_{\delta,\gamma,w}^{11} \quad (3r_D r_T^2 N_v) \quad (2928)$$

$$\tau_{\gamma,\delta,w}^{11} = \sum_{\epsilon \in A} Z_{\epsilon,\gamma} \tau_{\epsilon,\delta,w}^{10} \quad (2r_D r_T^3) \quad (2941)$$

Raw expression

$${}^{21}R_{a,\epsilon} \leftarrow \sum_{\gamma \in A} \sum_{i \in O} \sum_{j \in O} \sum_{k \in O} \sum_{l \in O} \sum_{b \in V} \sum_{c \in V} \sum_{d \in V} \frac{1}{4} Y_{i,\epsilon}^{2,*} Z_{\epsilon,\gamma}^* Y_{b,\gamma}^{3,*} Y_{j,\gamma}^{4,*} {}^2D_{a,i,b,j} {}^2T_{b,l,d,j} {}^2T_{c,k,a,i} V_{k,d,l,c} \quad (2929)$$

Factorized expression

$$\tau_{\gamma,\delta,w}^0 = \sum_{i \in O} {}^2D_{i,w}^2 Y_{i,\gamma}^4 Y_{i,\delta}^{2,*} \quad (3r_D r_T^2 N_o) \quad (2930)$$

$$\tau_{\gamma,\delta,w}^1 = \sum_{a \in V} {}^2D_{a,w}^3 Y_{a,\gamma}^1 Y_{a,\delta}^{3,*} \quad (3r_D r_T^2 N_v) \quad (2931)$$

$$\tau_{\gamma,\alpha}^2 = \sum_{a \in V} W_{a,\alpha}^4 Y_{a,\gamma}^1 \quad (2r_T r_V N_v) \quad (2932)$$

$$\tau_{\gamma,\alpha,i}^3 = \sum_{\beta \in B} X_{\alpha,\beta} W_{i,\beta}^3 \tau_{\gamma,\beta}^2 \quad (3r_T r_V^2 N_o) \quad (2933)$$

$$\tau_{\gamma,\alpha}^4 = \sum_{i \in O} W_{i,\alpha}^1 Y_{i,\gamma}^2 \quad (2r_T r_V N_o) \quad (2934)$$

$${}^{21}R_{a,\gamma} \leftarrow \sum_{\delta \in A} \sum_{w \in D} \frac{1}{4} {}^2D_{a,w}^1 Y_{a,\delta}^3 \tau_{\delta,\gamma,w}^0 \tau_{\delta,\gamma,w}^{11} \quad (4r_D r_T^2 N_v) \quad (2942)$$

Raw expression

$${}^{21}R_{a,\epsilon} \leftarrow \sum_{\gamma \in A} \sum_{i \in O} \sum_{j \in O} \sum_{k \in O} \sum_{l \in O} \sum_{b \in V} \sum_{c \in V} \sum_{d \in V} \frac{1}{4} Y_{i,\epsilon}^{2,*} Z_{\epsilon,\gamma}^* Y_{b,\gamma}^{3,*} Y_{j,\gamma}^{4,*} {}^2D_{a,i,b,j} {}^2T_{c,i,a,k} {}^2T_{d,j,b,l} V_{k,c,l,d} \quad (2943)$$

Factorized expression

$$\tau_{\gamma,\delta,w}^0 = \sum_{a \in V} {}^2D_{a,w}^3 Y_{a,\gamma}^3 Y_{a,\delta}^{3,*} \quad (3r_D r_T^2 N_v) \quad (2944)$$

$$\tau_{\gamma,\alpha}^1 = \sum_{a \in V} W_{a,\alpha}^4 Y_{a,\gamma}^1 \quad (2r_T r_V N_v) \quad (2945)$$

$$\tau_{\gamma,\alpha,i}^2 = \sum_{\delta \in A} Y_{i,\delta}^2 Z_{\delta,\gamma} \tau_{\delta,\alpha}^1 \quad (3r_T^2 r_V N_o) \quad (2946)$$

$$\tau_{\gamma,\alpha}^3 = \sum_{i \in O} W_{i,\alpha}^3 Y_{i,\gamma}^4 \quad (2r_T r_V N_o) \quad (2947)$$

$$\tau^4_{\gamma,\alpha,w} = \sum_{\delta \in A} \sum_{i \in O} {}^2D^4_{i,w} Y^{4,*}_{i,\gamma} \tau^3_{\delta,\alpha} \tau^0_{\delta,\gamma,w} \tau^2_{\delta,\alpha,i} \quad (5r_D r_T^2 r_V N_o^2)_{\delta,w} = \sum_{i \in O} {}^2D^4_{i,w} Y^4_{i,\gamma} Y^{4,*}_{i,\delta} \quad (3r_D r_T^2 N_o) \quad (2948)$$

$$\tau^5_{\gamma,\alpha,w} = \sum_{\beta \in B} X_{\alpha,\beta} \tau^4_{\gamma,\beta,w} \quad (2r_D r_T r_V^2) \quad (2949)$$

$$\tau^6_{\gamma,\alpha,w} = \sum_{\delta \in A} Z^*_{\gamma,\delta} \tau^5_{\delta,\alpha,w} \quad (2r_D r_T^2 r_V) \quad (2950)$$

$$\tau^7_{\gamma,\alpha} = \sum_{a \in V} W^2_{a,\alpha} Y^1_{a,\gamma} \quad (2r_T r_V N_v) \quad (2951)$$

$$\tau^8_{\gamma,\alpha,i} = \sum_{\delta \in A} Y^2_{i,\delta} Z_{\delta,\gamma} \tau^7_{\delta,\alpha} \quad (3r_T^2 r_V N_o) \quad (2952)$$

$$\tau^9_{\gamma,\alpha} = \sum_{i \in O} W^1_{i,\alpha} Y^4_{i,\gamma} \quad (2r_T r_V N_o) \quad (2953)$$

$$\tau^{10}_{\gamma,\delta,w,i} = \sum_{\alpha \in B} \tau^9_{\gamma,\alpha} \tau^6_{\delta,\alpha,w} \tau^8_{\gamma,\alpha,i} \quad (3r_D r_T^2 r_V N_o) \quad (2954)$$

$$\tau^{11}_{\gamma,\delta,w} = \sum_{i \in O} {}^2D^2_{i,w} Y^{2,*}_{i,\delta} \tau^{10}_{\gamma,\delta,w,i} \quad (3r_D r_T^2 N_o) \quad (2955)$$

$${}^{21}R_{a,\gamma} \leftarrow \sum_{\delta \in A} \sum_{w \in D} \frac{1}{4} {}^2D^1_{a,w} Y^3_{a,\delta} \tau^{11}_{\delta,\gamma,w} \quad (3r_D r_T^2 N_v) \quad (2956)$$

Raw expression

$${}^{21}R_{a,\epsilon} \leftarrow \sum_{\gamma \in A} \sum_{i \in O} \sum_{j \in O} \sum_{k \in O} \sum_{l \in O} \sum_{b \in V} \sum_{c \in V} \sum_{d \in V} \frac{1}{4} Y^{2,*}_{i,\epsilon} Z^*_{\epsilon,\gamma} Y^{3,*}_{b,\gamma} Y^{4,*}_{j,\gamma} {}^2D^{a,i,b,j} T_{c,i,a,k} {}^2T_{d,l,b,j} V_{k,d,l,c} \quad (2957)$$

Factorized expression

$$\tau^0_{\gamma,\delta,w} = \sum_{i \in O} {}^2D^2_{i,w} Y^2_{i,\gamma} Y^{2,*}_{i,\delta} \quad (3r_D r_T^2 N_o) \quad (2958)$$

$$\tau^1_{\gamma,\delta,w} = \sum_{a \in V} {}^2D^3_{a,w} Y^3_{a,\gamma} Y^{3,*}_{a,\delta} \quad (3r_D r_T^2 N_v) \quad (2959)$$

$$\tau^3_{\gamma,\delta,w} = \sum_{\epsilon \in A} Z^*_{\delta,\epsilon} \tau^1_{\gamma,\epsilon,w} \tau^2_{\gamma,\epsilon,w} \quad (3r_D r_T^3) \quad (2961)$$

$$\tau^4_{\gamma,\delta,w} = \sum_{\epsilon \in A} Z_{\gamma,\epsilon} \tau^3_{\epsilon,\delta,w} \quad (2r_D r_T^3) \quad (2962)$$

$$\tau^5_{\gamma,\alpha} = \sum_{a \in V} W^4_{a,\alpha} Y^1_{a,\gamma} \quad (2r_T r_V N_v) \quad (2963)$$

$$\tau^6_{\gamma,\alpha,i} = \sum_{\beta \in B} X_{\alpha,\beta} W^3_{i,\beta} \tau^5_{\gamma,\beta} \quad (3r_T r_V^2 N_o) \quad (2964)$$

$$\tau^7_{\gamma,\alpha} = \sum_{i \in O} W^1_{i,\alpha} Y^2_{i,\gamma} \quad (2r_T r_V N_o) \quad (2965)$$

$$\tau^8_{\gamma,\alpha} = \sum_{\delta \in A} \sum_{i \in O} Z_{\delta,\gamma} Y^4_{i,\gamma} \tau^7_{\delta,\alpha} \tau^6_{\delta,\alpha,i} \quad (4r_T^2 r_V N_o) \quad (2966)$$

$$\tau^9_{\gamma,a} = \sum_{\alpha \in B} W^2_{a,\alpha} \tau^8_{\gamma,\alpha} \quad (2r_T r_V N_v) \quad (2967)$$

$$\tau^{10}_{a,b} = \sum_{\gamma \in A} Y^3_{b,\gamma} \tau^9_{\gamma,a} \quad (2r_T N_v^2) \quad (2968)$$

$$\tau^{11}_{\gamma,a} = \sum_{b \in V} Y^1_{b,\gamma} \tau^{10}_{b,a} \quad (2r_T N_v^2) \quad (2969)$$

$${}^{21}R_{a,\gamma} \leftarrow \sum_{\delta \in A} \sum_{w \in D} \frac{1}{4} {}^2D^1_{a,w} \tau^{11}_{\delta,a} \tau^0_{\delta,\gamma,w} \tau^4_{\delta,\gamma,w} \quad (4r_D r_T^2 N_v) \quad (2970)$$

Raw expression

$${}^{21}R_{a,\epsilon} \leftarrow \sum_{\gamma \in A} \sum_{i \in O} \sum_{j \in O} \sum_{k \in O} \sum_{l \in O} \sum_{b \in V} \sum_{c \in V} \sum_{d \in V} \frac{1}{4} Y^{2,*}_{i,\epsilon} Z^*_{\epsilon,\gamma} Y^{3,*}_{b,\gamma} Y^{4,*}_{j,\gamma} {}^2D^{a,i,b,j} T_{c,j,a,i} {}^2T_{d,k,b,l} V_{k,c,l,d} \quad (2971)$$

Factorized expression

$$\tau^0_{\gamma,\delta,w} = \sum_{i \in O} {}^2D^2_{i,w} Y^4_{i,\gamma} Y^{2,*}_{i,\delta} \quad (3r_D r_T^2 N_o) \quad (2972)$$

$$\tau^1_{\gamma,\delta,w} = \sum_{a \in V} {}^2D^3_{a,w} Y^3_{a,\gamma} Y^{3,*}_{a,\delta} \quad (3r_D r_T^2 N_v) \quad (2973)$$

$$\tau^0_{\gamma,\delta,w} = \sum_{i \in O} {}^2D^2_{i,w} Y^4_{i,\gamma} Y^{2,*}_{i,\delta} \quad (3r_D r_T^2 N_o) \quad (2986)$$

$$\tau^2_{\gamma,\alpha} = \sum_{a \in V} W^4_{a,\alpha} Y^1_{a,\gamma} \quad (2r_T r_V N_v) \quad (2974)$$

$$\tau^1_{\gamma,\delta,w} = \sum_{i \in O} {}^2D^4_{i,w} Y^2_{i,\gamma} Y^{4,*}_{i,\delta} \quad (3r_D r_T^2 N_o) \quad (2987)$$

$$\tau^3_{\gamma,\alpha,i} = \sum_{\beta \in B} X_{\alpha,\beta} W^3_{i,\beta} \tau^2_{\gamma,\beta} \quad (3r_T r_V^2 N_o) \quad (2975)$$

$$\tau^2_{\gamma,\alpha} = \sum_{a \in V} W^4_{a,\alpha} Y^1_{a,\gamma} \quad (2r_T r_V N_v) \quad (2988)$$

$$\tau^4_{\gamma,\alpha} = \sum_{i \in O} W^1_{i,\alpha} Y^2_{i,\gamma} \quad (2r_T r_V N_o) \quad (2976)$$

$$\tau^3_{\gamma,\alpha,i} = \sum_{\beta \in B} X_{\alpha,\beta} W^3_{i,\beta} \tau^2_{\gamma,\beta} \quad (3r_T r_V^2 N_o) \quad (2989)$$

$$\tau^5_{\gamma,\alpha} = \sum_{a \in V} W^2_{a,\alpha} Y^1_{a,\gamma} \quad (2r_T r_V N_v) \quad (2977)$$

$$\tau^4_{\gamma,\alpha} = \sum_{i \in O} W^1_{i,\alpha} Y^2_{i,\gamma} \quad (2r_T r_V N_o) \quad (2990)$$

$$\tau^6_{\gamma,\delta,i} = \sum_{\alpha \in B} \tau^4_{\gamma,\alpha} \tau^5_{\delta,\alpha} \tau^3_{\gamma,\alpha,i} \quad (3r_T^2 r_V N_o) \quad (2978)$$

$$\tau^5_{\gamma,\alpha} = \sum_{\delta \in A} \sum_{i \in O} Z_{\delta,\gamma} Y^4_{i,\gamma} \tau^4_{\delta,\alpha} \tau^3_{\delta,\alpha,i} \quad (4r_T^2 r_V N_o) \quad (2991)$$

$$\tau^7_{\gamma,\delta,\epsilon} = \sum_{i \in O} Z_{\delta,\epsilon} Y^4_{i,\epsilon} \tau^6_{\gamma,\delta,i} \quad (3r_T^3 N_o) \quad (2979)$$

$$\tau^6_{\gamma,a} = \sum_{\alpha \in B} W^2_{a,\alpha} \tau^5_{\gamma,\alpha} \quad (2r_T r_V N_v) \quad (2992)$$

$$\tau^8_{\gamma,\delta,i} = \sum_{\epsilon \in A} Y^2_{i,\epsilon} \tau^7_{\gamma,\epsilon,\delta} \quad (2r_T^3 N_o) \quad (2980)$$

$$\tau^7_{a,b} = \sum_{\gamma \in A} Y^3_{b,\gamma} \tau^6_{\gamma,a} \quad (2r_T N_v^2) \quad (2993)$$

$$\tau^9_{\gamma,\delta,w} = \sum_{\epsilon \in A} \sum_{i \in O} {}^2D^4_{i,w} Y^{4,*}_{i,\delta} \tau^1_{\epsilon,\delta,w} \tau^8_{\gamma,\epsilon,i} \quad (4r_D r_T^3 N_o) \quad (2981)$$

$$\tau^8_{\gamma,a} = \sum_{b \in V} Y^1_{b,\gamma} \tau^7_{b,a} \quad (2r_T N_v^2) \quad (2994)$$

$$\tau^{10}_{\gamma,\delta,w} = \sum_{\epsilon \in A} Z^*_{\delta,\epsilon} \tau^9_{\gamma,\epsilon,w} \quad (2r_D r_T^3) \quad (2982)$$

$$\tau^9_{\gamma,\delta,w} = \sum_{a \in V} {}^2D^3_{a,w} Y^{3,*}_{a,\delta} \tau^8_{\gamma,a} \quad (3r_D r_T^2 N_v) \quad (2995)$$

$$\tau^{11}_{\gamma,\delta,w} = \sum_{\epsilon \in A} Z_{\epsilon,\gamma} \tau^{10}_{\epsilon,\delta,w} \quad (2r_D r_T^3) \quad (2983)$$

$$\tau^{10}_{\gamma,\delta,w} = \sum_{\epsilon \in A} Z^*_{\delta,\epsilon} \tau^1_{\gamma,\epsilon,w} \tau^9_{\gamma,\epsilon,w} \quad (3r_D r_T^3) \quad (2996)$$

$$\tau^{11}_{\gamma,\delta,w} = \sum_{\epsilon \in A} Z_{\epsilon,\gamma} \tau^{10}_{\epsilon,\delta,w} \quad (2r_D r_T^3) \quad (2997)$$

$${}^{21}R_{a,\gamma} \leftarrow \sum_{\delta \in A} \sum_{w \in D} \frac{1}{4} {}^2D^1_{a,w} Y^3_{a,\delta} \tau^0_{\delta,\gamma,w} \tau^{11}_{\delta,\gamma,w} \quad (4r_D r_T^2 N_v) \quad (2984)$$

$${}^{21}R_{a,\gamma} \leftarrow \sum_{\delta \in A} \sum_{w \in D} \frac{1}{4} {}^2D^1_{a,w} Y^3_{a,\delta} \tau^0_{\delta,\gamma,w} \tau^{11}_{\delta,\gamma,w} \quad (4r_D r_T^2 N_v) \quad (2998)$$

Raw expression

$${}^{21}R_{a,\epsilon} \leftarrow \sum_{\gamma \in A} \sum_{i \in O} \sum_{j \in O} \sum_{k \in O} \sum_{l \in O} \sum_{b \in V} \sum_{c \in V} \sum_{d \in V} \frac{1}{4} Y^{2,*}_{i,\epsilon} Z^*_{\epsilon,\gamma} Y^{3,*}_{b,\gamma} Y^{4,*}_{j,\gamma} {}^2D^{a,i,b,j} {}^2T_{c,j,a,k} {}^2T_{d,i,b,l} V_{k,d,l,c} \quad (2985)$$

Factorized expression

Raw expression

$${}^{21}R_{a,\epsilon} \leftarrow \sum_{\gamma \in A} \sum_{i \in O} \sum_{j \in O} \sum_{k \in O} \sum_{l \in O} \sum_{b \in V} \sum_{c \in V} \sum_{d \in V} \frac{1}{4} Y^{2,*}_{i,\epsilon} Z^*_{\epsilon,\gamma} Y^{3,*}_{b,\gamma} Y^{4,*}_{j,\gamma} {}^2D^{a,i,b,j} {}^2T_{c,k,a,i} {}^2T_{d,j,b,l} V_{k,d,l,c} \quad (2999)$$

Factorized expression

$$\tau^0_{\gamma,\delta,w} = \sum_{a \in V} {}^2D^3_{a,w} Y^3_{a,\gamma} Y^{3,*}_{a,\delta} \quad (3r_D r_T^2 N_v) \quad (3000)$$

$$\tau^1_{\gamma,\delta,w} = \sum_{i \in O} {}^2D^4_{i,w} Y^4_{i,\gamma} Y^{4,*}_{i,\delta} \quad (3r_D r_T^2 N_o) \quad (3001)$$

$$\tau^2_{\gamma,\delta,w} = \sum_{\epsilon \in A} Z^*_{\delta,\epsilon} \tau^0_{\gamma,\epsilon,w} \tau^1_{\gamma,\epsilon,w} \quad (3r_D r_T^3) \quad (3002)$$

$$\tau^3_{\gamma,\delta,w} = \sum_{\epsilon \in A} Z_{\gamma,\epsilon} \tau^2_{\epsilon,\delta,w} \quad (2r_D r_T^3) \quad (3003)$$

$$\tau^4_{\gamma,\alpha} = \sum_{a \in V} W^2_{a,\alpha} Y^1_{a,\gamma} \quad (2r_T r_V N_v) \quad (3004)$$

$$\tau^5_{\gamma,\alpha,i} = \sum_{\beta \in B} W^1_{i,\beta} X_{\beta,\alpha} \tau^4_{\gamma,\beta} \quad (3r_T r_V^2 N_o) \quad (3005)$$

$$\tau^6_{\gamma,\alpha} = \sum_{i \in O} W^3_{i,\alpha} Y^2_{i,\gamma} \quad (2r_T r_V N_o) \quad (3006)$$

$$\tau^7_{\gamma,\alpha} = \sum_{a \in V} W^4_{a,\alpha} Y^1_{a,\gamma} \quad (2r_T r_V N_v) \quad (3007)$$

$$\tau^8_{\gamma,\delta,i} = \sum_{\alpha \in B} \tau^6_{\gamma,\alpha} \tau^7_{\delta,\alpha} \tau^5_{\gamma,\alpha,i} \quad (3r_T^2 r_V N_o) \quad (3008)$$

$$\tau^9_{\gamma,\delta,\epsilon} = \sum_{i \in O} Z_{\delta,\epsilon} Y^4_{i,\epsilon} \tau^8_{\gamma,\delta,i} \quad (3r_T^3 N_o) \quad (3009)$$

$$\tau^{10}_{\gamma,\delta,i} = \sum_{\epsilon \in A} Y^2_{i,\epsilon} \tau^9_{\gamma,\epsilon,\delta} \quad (2r_T^3 N_o) \quad (3010)$$

$$\tau^{11}_{\gamma,\delta,w} = \sum_{\epsilon \in A} \sum_{i \in O} {}^2D^2_{i,w} Y^{2,*}_{i,\delta} \tau^{10}_{\epsilon,\gamma,i} \tau^3_{\epsilon,\delta,w} \quad (4r_D r_T^3 N_o) \quad (3011)$$

$${}^{21}R_{a,\gamma} \leftarrow \sum_{\delta \in A} \sum_{w \in D} \frac{1}{4} {}^2D^1_{a,w} Y^3_{a,\delta} \tau^{11}_{\delta,\gamma,w} \quad (3r_D r_T^2 N_v) \quad (3012)$$

Raw expression

$${}^{21}R_{a,\epsilon} \leftarrow \sum_{\gamma \in A} \sum_{i \in O} \sum_{j \in O} \sum_{k \in O} \sum_{l \in O} \sum_{b \in V} \sum_{c \in V} \sum_{d \in V} \frac{1}{4} Y^{2,*}_{i,\epsilon} Z^*_{\epsilon,\gamma} Y^{3,*}_{b,\gamma} Y^{4,*}_{j,\gamma} {}^2D^{a,i,b,j}_{c,k,a,l} {}^2T_{d,i,b,j} V_{k,d,l,c} \quad (3013)$$

Factorized expression

$$\tau^0_{\gamma,\alpha} = \sum_{a \in V} W^2_{a,\alpha} Y^1_{a,\gamma} \quad (2r_T r_V N_v) \quad (3014)$$

$$\tau^1_{\gamma,\alpha,i} = \sum_{\beta \in B} W^1_{i,\beta} X_{\beta,\alpha} \tau^0_{\gamma,\beta} \quad (3r_T r_V^2 N_o) \quad (3015)$$

$$\tau^2_{\gamma,\delta,\alpha} = \sum_{i \in O} Y^4_{i,\delta} \tau^1_{\gamma,\alpha,i} \quad (2r_T^2 r_V N_o) \quad (3016)$$

$$\tau^3_{\gamma,\alpha} = \sum_{a \in V} W^4_{a,\alpha} Y^1_{a,\gamma} \quad (2r_T r_V N_v) \quad (3017)$$

$$\tau^4_{\gamma,\alpha,i} = \sum_{\delta \in A} Y^2_{i,\delta} Z_{\delta,\gamma} \tau^3_{\delta,\alpha} \quad (3r_T^2 r_V N_o) \quad (3018)$$

$$\tau^5_{\gamma,\delta,\alpha,w} = \sum_{i \in O} {}^2D^4_{i,w} Y^{4,*}_{i,\delta} \tau^4_{\gamma,\alpha,i} \quad (3r_D r_T^2 r_V N_o) \quad (3019)$$

$$\tau^6_{\gamma,\delta,w} = \sum_{a \in V} {}^2D^3_{a,w} Y^3_{a,\gamma} Y^{3,*}_{a,\delta} \quad (3r_D r_T^2 N_v) \quad (3020)$$

$$\tau^7_{\gamma,\delta,w,i} = \sum_{\epsilon \in A} Z_{\gamma,\epsilon} Y^4_{i,\epsilon} \tau^6_{\epsilon,\delta,w} \quad (3r_D r_T^3 N_o) \quad (3021)$$

$$\tau^8_{\gamma,\delta,\alpha,w} = \sum_{i \in O} W^3_{i,\alpha} \tau^7_{\gamma,\delta,w,i} \quad (2r_D r_T^2 r_V N_o) \quad (3022)$$

$$\tau^9_{\gamma,\delta,\epsilon,w} = \sum_{\alpha \in B} \tau^2_{\gamma,\delta,\alpha} \tau^5_{\delta,\epsilon,\alpha,w} \tau^8_{\gamma,\epsilon,\alpha,w} \quad (3r_D r_T^3 r_V) \quad (3023)$$

$$\tau^{10}_{\gamma,\delta,w,i} = \sum_{\epsilon \in A} {}^2D^2_{i,w} Y^2_{i,\epsilon} \tau^9_{\epsilon,\gamma,\delta,w} \quad (3r_D r_T^3 N_o) \quad (3024)$$

$$\tau^{11}_{\gamma,\delta,w} = \sum_{\epsilon \in A} \sum_{i \in O} Y^{2,*}_{i,\delta} Z^*_{\delta,\epsilon} \tau^{10}_{\gamma,\epsilon,w,i} \quad (3r_D r_T^3 N_o) \quad (3025)$$

$${}^{21}R_{a,\gamma} \leftarrow \sum_{\delta \in A} \sum_{w \in D} \frac{1}{4} {}^2D^1_{a,w} Y^3_{a,\delta} \tau^{11}_{\delta,\gamma,w} \quad (3r_D r_T^2 N_v) \quad (3026)$$

### VIII. THC-RCCSD DOUBLES ( $Y^2$ FACTOR) EQUATION

Here expressions for a THC-RCCSD doubles residual, projected against all factors except  $Y^2$ , are given along with their cost

#### A. Contributions from $H$

Raw expression

$${}^2R^2_{i,\epsilon} \leftarrow \sum_{\gamma \in A} \sum_{j \in O} \sum_{a \in V} \sum_{b \in V} Y^{1,*}_{a,\epsilon} Z^*_{\epsilon,\gamma} Y^{3,*}_{b,\gamma} Y^{4,*}_{j,\gamma} {}^2D^{a,i,b,j}_{V_{a,i,b,j}} \quad (3027)$$

Factorized expression

$$\tau^0_{\gamma,\alpha,w} = \sum_{a \in V} {}^2D^1_{a,w} W^1_{a,\alpha} Y^{1,*}_{a,\gamma} \quad (3r_D r_T r_V N_v) \quad (3028)$$

$$\tau^1_{\gamma,\alpha,w} = \sum_{a \in V} {}^2D^3_{a,w} W^3_{a,\alpha} Y^{3,*}_{a,\gamma} \quad (3r_D r_T r_V N_v) \quad (3029)$$

$$\tau^2_{\gamma,\alpha,w} = \sum_{i \in O} {}^2D^4_{i,w} W^4_{i,\alpha} Y^{4,*}_{i,\gamma} \quad (3r_D r_T r_V N_o) \quad (3030)$$

$$\tau^3_{\gamma,\alpha,w} = \sum_{\beta \in B} X_{\alpha,\beta} \tau^1_{\gamma,\beta,w} \tau^2_{\gamma,\beta,w} \quad (3r_D r_T r_V^2) \quad (3031)$$

$$\tau^4_{\gamma,\alpha,w} = \sum_{\delta \in A} Z^*_{\gamma,\delta} \tau^3_{\delta,\alpha,w} \quad (2r_D r_T^2 r_V) \quad (3032)$$

$$\tau^5_{\gamma,w,i} = \sum_{\alpha \in B} W^2_{i,\alpha} \tau^0_{\gamma,\alpha,w} \tau^4_{\gamma,\alpha,w} \quad (3r_D r_T r_V N_o) \quad (3033)$$

$${}^2R^2_{i,\gamma} \leftarrow \sum_{w \in D} {}^2D^2_{i,w} \tau^5_{\gamma,w,i} \quad (2r_D r_T N_o) \quad (3034)$$

#### B. Contributions from $(H^1 T)_c$

Raw expression

$${}^2R^2_{i,\epsilon} \leftarrow \sum_{\gamma \in A} \sum_{j \in O} \sum_{a \in V} \sum_{b \in V} \sum_{c \in V} {}^1T_{c,i} Y^{1,*}_{a,\epsilon} Z^*_{\epsilon,\gamma} Y^{3,*}_{b,\gamma} Y^{4,*}_{j,\gamma} {}^2D^{a,i,b,j}_{V_{a,c,b,j}} \quad (3035)$$

Factorized expression

$$\tau^0_{\gamma,\alpha,w} = \sum_{a \in V} {}^2D^3_{a,w} W^1_{a,\alpha} Y^{3,*}_{a,\gamma} \quad (3r_D r_T r_V N_v) \quad (3036)$$

$$\tau^1_{\gamma,\alpha,w} = \sum_{i \in O} {}^2D^4_{i,w} W^2_{i,\alpha} Y^{4,*}_{i,\gamma} \quad (3r_D r_T r_V N_o) \quad (3037)$$

$$\tau^2_{\gamma,\alpha,w} = \sum_{\beta \in B} X_{\beta,\alpha} \tau^0_{\gamma,\beta,w} \tau^1_{\gamma,\beta,w} \quad (3r_D r_T r_V^2) \quad (3038)$$

$$\tau^3_{\gamma,\alpha,w} = \sum_{\delta \in A} Z^*_{\gamma,\delta} \tau^2_{\delta,\alpha,w} \quad (2r_D r_T^2 r_V) \quad (3039)$$

$$\tau^4_{\gamma,w,i} = \sum_{a \in V} {}^2D^1_{a,w} {}^1T_{a,i} Y^{1,*}_{a,\gamma} \quad (3r_D r_T N_o N_v) \quad (3040)$$

$$\tau^5_{\gamma,\alpha,w} = \sum_{i \in O} W^3_{i,\alpha} \tau^4_{\gamma,w,i} \quad (2r_D r_T r_V N_o) \quad (3041)$$

$$\tau^6_{\gamma,w,i} = \sum_{\alpha \in B} W^4_{i,\alpha} \tau^3_{\gamma,\alpha,w} \tau^5_{\gamma,\alpha,w} \quad (3r_D r_T r_V N_o) \quad (3042)$$

$${}^2R^2_{i,\gamma} \leftarrow - \sum_{w \in D} {}^2D^2_{i,w} \tau^6_{\gamma,w,i} \quad (2r_D r_T N_o) \quad (3043)$$

Raw expression

$${}^2R^2_{i,\epsilon} \leftarrow \sum_{\gamma \in A} \sum_{j \in O} \sum_{a \in V} \sum_{b \in V} \sum_{c \in V} {}^1T_{c,j} Y^{1,*}_{a,\epsilon} Z^*_{\epsilon,\gamma} Y^{3,*}_{b,\gamma} Y^{4,*}_{j,\gamma} {}^2D^{a,i,b,j}_{V_{a,i,b,c}} \quad (3044)$$

Factorized expression

$$\tau^0_{\gamma,\alpha,w} = \sum_{a \in V} {}^2D^1_{a,w} W^1_{a,\alpha} Y^{1,*}_{a,\gamma} \quad (3r_D r_T r_V N_v) \quad (3045)$$

$$\tau^1_{\gamma,w,i} = \sum_{a \in V} {}^2D^3_{a,w} {}^1T_{a,i} Y^{3,*}_{a,\gamma} \quad (3r_D r_T N_o N_v) \quad (3046)$$

$$\tau^2_{\gamma,\alpha,w} = \sum_{i \in O} W^3_{i,\alpha} \tau^1_{\gamma,w,i} \quad (2r_D r_T r_V N_o) \quad (3047)$$



$$\tau^3_{\gamma,\alpha,w} = \sum_{i \in O} {}^2D^4_{i,w} W^4_{i,\alpha} Y^{4,*}_{i,\gamma} \quad (3r_D r_T r_V N_o) \quad (3048)$$

$$\tau^4_{\gamma,\alpha,w} = \sum_{\beta \in B} X_{\alpha,\beta} \tau^2_{\gamma,\beta,w} \tau^3_{\gamma,\beta,w} \quad (3r_D r_T r_V^2) \quad (3049)$$

$$\tau^5_{\gamma,\alpha,w} = \sum_{\delta \in A} Z^*_{\gamma,\delta} \tau^4_{\delta,\alpha,w} \quad (2r_D r_T^2 r_V) \quad (3050)$$

$$\tau^6_{\gamma,w,i} = \sum_{\alpha \in B} W^2_{i,\alpha} \tau^0_{\gamma,\alpha,w} \tau^5_{\gamma,\alpha,w} \quad (3r_D r_T r_V N_o) \quad (3051)$$

$${}^2R^2_{i,\gamma} \leftarrow - \sum_{w \in D} {}^2D^2_{i,w} \tau^6_{\gamma,w,i} \quad (2r_D r_T N_o) \quad (3052)$$

Raw expression

$${}^2R^2_{i,\epsilon} \leftarrow - \sum_{\gamma \in A} \sum_{j \in O} \sum_{k \in O} \sum_{a \in V} \sum_{b \in V} {}^1T_{a,k} Y^{1,*}_{a,\epsilon} \quad (3053)$$

$$Z^*_{\epsilon,\gamma} Y^{3,*}_{b,\gamma} Y^{4,*}_{j,\gamma} {}^2D^{a,i,b,j} V_{b,j,k,i}$$

Factorized expression

$$\tau^0_{\gamma,\alpha,w} = \sum_{a \in V} {}^2D^1_{a,w} W^1_{a,\alpha} Y^{1,*}_{a,\gamma} \quad (3r_D r_T r_V N_v) \quad (3054)$$

$$\tau^1_{\gamma,\alpha,w} = \sum_{a \in V} {}^2D^3_{a,w} W^3_{a,\alpha} Y^{3,*}_{a,\gamma} \quad (3r_D r_T r_V N_v) \quad (3055)$$

$$\tau^2_{\gamma,\alpha,w} = \sum_{i \in O} {}^2D^4_{i,w} W^4_{i,\alpha} Y^{4,*}_{i,\gamma} \quad (3r_D r_T r_V N_o) \quad (3056)$$

$$\tau^3_{\gamma,\alpha,w} = \sum_{\beta \in B} X_{\alpha,\beta} \tau^1_{\gamma,\beta,w} \tau^2_{\gamma,\beta,w} \quad (3r_D r_T r_V^2) \quad (3057)$$

$$\tau^4_{\gamma,\alpha,w} = \sum_{\delta \in A} Z^*_{\gamma,\delta} \tau^3_{\delta,\alpha,w} \quad (2r_D r_T^2 r_V) \quad (3058)$$

$$\tau^5_{\alpha,i} = \sum_{a \in V} {}^1T_{a,i} W^2_{a,\alpha} \quad (2r_V N_o N_v) \quad (3059)$$

$$\tau^6_{\gamma,w,i} = \sum_{\alpha \in B} \tau^5_{\alpha,i} \tau^0_{\gamma,\alpha,w} \tau^4_{\gamma,\alpha,w} \quad (3r_D r_T r_V N_o) \quad (3060)$$

$${}^2R^2_{i,\gamma} \leftarrow \sum_{w \in D} {}^2D^2_{i,w} \tau^6_{\gamma,w,i} \quad (2r_D r_T N_o) \quad (3061)$$

Raw expression

$${}^2R^2_{i,\epsilon} \leftarrow - \sum_{\gamma \in A} \sum_{j \in O} \sum_{k \in O} \sum_{a \in V} \sum_{b \in V} {}^1T_{b,k} Y^{1,*}_{a,\epsilon} \quad (3062)$$

$$Z^*_{\epsilon,\gamma} Y^{3,*}_{b,\gamma} Y^{4,*}_{j,\gamma} {}^2D^{a,i,b,j} V_{a,i,k,j}$$

Factorized expression

$$\tau^0_{\gamma,\alpha,w} = \sum_{a \in V} {}^2D^1_{a,w} W^1_{a,\alpha} Y^{1,*}_{a,\gamma} \quad (3r_D r_T r_V N_v) \quad (3063)$$

$$\tau^1_{\alpha,i} = \sum_{a \in V} {}^1T_{a,i} W^4_{a,\alpha} \quad (2r_V N_o N_v) \quad (3064)$$

$$\tau^2_{\gamma,\alpha,w} = \sum_{i \in O} {}^2D^4_{i,w} Y^{4,*}_{i,\gamma} \tau^1_{\alpha,i} \quad (3r_D r_T r_V N_o) \quad (3065)$$

$$\tau^3_{\gamma,\alpha,w} = \sum_{a \in V} {}^2D^3_{a,w} W^3_{a,\alpha} Y^{3,*}_{a,\gamma} \quad (3r_D r_T r_V N_v) \quad (3066)$$

$$\tau^4_{\gamma,\alpha,w} = \sum_{\beta \in B} X_{\alpha,\beta} \tau^2_{\gamma,\beta,w} \tau^3_{\gamma,\beta,w} \quad (3r_D r_T r_V^2) \quad (3067)$$

$$\tau^5_{\gamma,\alpha,w} = \sum_{\delta \in A} Z^*_{\gamma,\delta} \tau^4_{\delta,\alpha,w} \quad (2r_D r_T^2 r_V) \quad (3068)$$

$$\tau^6_{\gamma,w,i} = \sum_{\alpha \in B} W^2_{i,\alpha} \tau^0_{\gamma,\alpha,w} \tau^5_{\gamma,\alpha,w} \quad (3r_D r_T r_V N_o) \quad (3069)$$

$${}^2R^2_{i,\gamma} \leftarrow \sum_{w \in D} {}^2D^2_{i,w} \tau^6_{\gamma,w,i} \quad (2r_D r_T N_o) \quad (3070)$$

### C. Contributions from $(H^1 T^1 T)_c$

Raw expression

$${}^2R^2_{i,\epsilon} \leftarrow - \sum_{\gamma \in A} \sum_{j \in O} \sum_{k \in O} \sum_{a \in V} \sum_{b \in V} \sum_{c \in V} {}^1T_{a,k} {}^1T_{c,i} Y^{1,*}_{a,\epsilon} Z^*_{\epsilon,\gamma} Y^{3,*}_{b,\gamma} Y^{4,*}_{j,\gamma} {}^2D^{a,i,b,j} V_{b,j,k,c} \quad (3071)$$

Factorized expression

$$\tau^0_{\gamma,\alpha,w} = \sum_{a \in V} {}^2D^1_{a,w} W^1_{a,\alpha} Y^{1,*}_{a,\gamma} \quad (3r_D r_T r_V N_v) \quad (3072)$$

$$\tau^1_{\alpha,i} = \sum_{a \in V} {}^1T_{a,i} W^4_{a,\alpha} \quad (2r_V N_o N_v) \quad (3073)$$

$$\tau^2_{\gamma,\alpha,w} = \sum_{i \in O} {}^2D^4_{i,w} Y^{4,*}_{i,\gamma} \tau^1_{\alpha,i} \quad (3r_D r_T r_V N_o) \quad (3074)$$

$$\tau^3_{\gamma,\alpha,w} = \sum_{a \in V} {}^2D^3_{a,w} W^3_{a,\alpha} Y^{3,*}_{a,\gamma} \quad (3r_D r_T r_V N_v) \quad (3075)$$

$$\tau^4_{\gamma,\alpha,w} = \sum_{\beta \in B} X_{\alpha,\beta} \tau^2_{\gamma,\beta,w} \tau^3_{\gamma,\beta,w} \quad (3r_D r_T r_V^2) \quad (3076)$$

$$\tau^5_{\gamma,\alpha,w} = \sum_{\delta \in A} Z^*_{\gamma,\delta} \tau^4_{\delta,\alpha,w} \quad (2r_D r_T^2 r_V) \quad (3077)$$

$$\tau^6_{\alpha,i} = \sum_{a \in V} {}^1T_{a,i} W^2_{a,\alpha} \quad (2r_V N_o N_v) \quad (3078)$$

$$\tau^7_{\gamma,w,i} = \sum_{\alpha \in B} \tau^6_{\alpha,i} \tau^0_{\gamma,\alpha,w} \tau^5_{\gamma,\alpha,w} \quad (3r_D r_T r_V N_o) \quad (3079)$$

$${}^2R^2_{i,\gamma} \leftarrow \sum_{w \in D} {}^2D^2_{i,w} \tau^7_{\gamma,w,i} \quad (2r_D r_T N_o) \quad (3080)$$

Raw expression

$${}^2R^2_{i,\epsilon} \leftarrow - \sum_{\gamma \in A} \sum_{j \in O} \sum_{k \in O} \sum_{a \in V} \sum_{b \in V} \sum_{c \in V} {}^1T_{a,k} {}^1T_{c,j} Y^{1,*}_{a,\epsilon} Z^*_{\epsilon,\gamma} Y^{3,*}_{b,\gamma} Y^{4,*}_{j,\gamma} {}^2D^{a,i,b,j} V_{b,c,k,i} \quad (3081)$$

Factorized expression

$$\tau^0_{\gamma,w,i} = \sum_{a \in V} {}^2D^3_{a,w} {}^1T_{a,i} Y^{3,*}_{a,\gamma} \quad (3r_D r_T N_o N_v) \quad (3082)$$

$$\tau^1_{\gamma,\alpha,w} = \sum_{i \in O} W^3_{i,\alpha} \tau^0_{\gamma,w,i} \quad (2r_D r_T r_V N_o) \quad (3083)$$

$$\tau^2_{\gamma,\alpha,w} = \sum_{i \in O} {}^2D^4_{i,w} W^4_{i,\alpha} Y^{4,*}_{i,\gamma} \quad (3r_D r_T r_V N_o) \quad (3084)$$

$$\tau^3_{\gamma,\alpha,w} = \sum_{\beta \in B} X_{\alpha,\beta} \tau^1_{\gamma,\beta,w} \tau^2_{\gamma,\beta,w} \quad (3r_D r_T r_V^2) \quad (3085)$$

$$\tau^4_{\gamma,\alpha,w} = \sum_{\delta \in A} Z^*_{\gamma,\delta} \tau^3_{\delta,\alpha,w} \quad (2r_D r_T^2 r_V) \quad (3086)$$

$$\tau^5_{\gamma,w,i} = \sum_{a \in V} {}^2D^1_{a,w} {}^1T_{a,i} Y^{1,*}_{a,\gamma} \quad (3r_D r_T N_o N_v) \quad (3087)$$

$$\tau^6_{\gamma,\alpha,w} = \sum_{i \in O} W^1_{i,\alpha} \tau^5_{\gamma,w,i} \quad (2r_D r_T r_V N_o) \quad (3088)$$

$$\tau^7_{\gamma,w,i} = \sum_{\alpha \in B} W^2_{i,\alpha} \tau^4_{\gamma,\alpha,w} \tau^6_{\gamma,\alpha,w} \quad (3r_D r_T r_V N_o) \quad (3089)$$

$${}^2R^2_{i,\gamma} \leftarrow \sum_{w \in D} {}^2D^2_{i,w} \tau^7_{\gamma,w,i} \quad (2r_D r_T N_o) \quad (3090)$$

Raw expression

$${}^2R^2_{i,\epsilon} \leftarrow - \sum_{\gamma \in A} \sum_{j \in O} \sum_{k \in O} \sum_{a \in V} \sum_{b \in V} \sum_{c \in V} {}^1T_{b,k} {}^1T_{c,i} Y^{1,*}_{a,\epsilon} Z^*_{\epsilon,\gamma} Y^{3,*}_{b,\gamma} Y^{4,*}_{j,\gamma} {}^2D^{a,i,b,j} V_{a,c,k,j} \quad (3091)$$

Factorized expression

$$\tau^0_{\gamma,\alpha,w} = \sum_{a \in V} {}^2D^3_{a,w} W^1_{a,\alpha} Y^{3,*}_{a,\gamma} \quad (3r_D r_T r_V N_v) \quad (3092)$$

$$\tau^1_{\gamma,\alpha,w} = \sum_{i \in O} {}^2D^4_{i,w} W^2_{i,\alpha} Y^{4,*}_{i,\gamma} \quad (3r_D r_T r_V N_o) \quad (3093)$$

$$\tau^2_{\gamma,\alpha,w} = \sum_{\beta \in B} X_{\beta,\alpha} \tau^0_{\gamma,\beta,w} \tau^1_{\gamma,\beta,w} \quad (3r_D r_T r_V^2) \quad (3094)$$

$$\tau^3_{\gamma,\alpha,w} = \sum_{\delta \in A} Z^*_{\gamma,\delta} \tau^2_{\delta,\alpha,w} \quad (2r_D r_T^2 r_V) \quad (3095)$$

$$\tau^4_{\gamma,w,i} = \sum_{a \in V} {}^2D^1_{a,w} {}^1T_{a,i} Y^{1,*}_{a,\gamma} \quad (3r_D r_T N_o N_v) \quad (3096)$$

$$\tau^5_{\gamma,\alpha,w} = \sum_{i \in O} W^3_{i,\alpha} \tau^4_{\gamma,w,i} \quad (2r_D r_T r_V N_o) \quad (3097)$$

$$\tau^6_{\alpha,i} = \sum_{a \in V} {}^1T_{a,i} W^4_{a,\alpha} \quad (2r_V N_o N_v) \quad (3098)$$

$$\tau^7_{\gamma,w,i} = \sum_{\alpha \in B} \tau^6_{\alpha,i} \tau^3_{\gamma,\alpha,w} \tau^5_{\gamma,\alpha,w} \quad (3r_D r_T r_V N_o) \quad (3099)$$

$${}^2R^2_{i,\gamma} \leftarrow - \sum_{w \in D} {}^2D^2_{i,w} \tau^7_{\gamma,w,i} \quad (2r_D r_T N_o) \quad (3100)$$

Raw expression

$${}^2R^2_{i,\epsilon} \leftarrow - \sum_{\gamma \in A} \sum_{j \in O} \sum_{k \in O} \sum_{a \in V} \sum_{b \in V} \sum_{c \in V} {}^1T_{b,k} {}^1T_{c,j} Y^{1,*}_{a,\epsilon} Z^*_{\epsilon,\gamma} Y^{3,*}_{b,\gamma} Y^{4,*}_{j,\gamma} {}^2D^{a,i,b,j}_{a,i,k,c} V_{a,i,k,c} \quad (3101)$$

Factorized expression

$$\tau^0_{\alpha,i} = \sum_{a \in V} {}^1T_{a,i} W^2_{a,\alpha} \quad (2r_V N_o N_v) \quad (3102)$$

$$\tau^1_{\gamma,\alpha,w} = \sum_{i \in O} {}^2D^4_{i,w} Y^{4,*}_{i,\gamma} \tau^0_{\alpha,i} \quad (3r_D r_T r_V N_o) \quad (3103)$$

$$\tau^2_{\gamma,\alpha,w} = \sum_{a \in V} {}^2D^3_{a,w} W^1_{a,\alpha} Y^{3,*}_{a,\gamma} \quad (3r_D r_T r_V N_v) \quad (3104)$$

$$\tau^3_{\gamma,\alpha,w} = \sum_{\beta \in B} X_{\beta,\alpha} \tau^1_{\gamma,\beta,w} \tau^2_{\gamma,\beta,w} \quad (3r_D r_T r_V^2) \quad (3105)$$

$$\tau^4_{\gamma,\alpha,w} = \sum_{\delta \in A} Z^*_{\gamma,\delta} \tau^3_{\delta,\alpha,w} \quad (2r_D r_T^2 r_V) \quad (3106)$$

$$\tau^5_{\gamma,w,i} = \sum_{a \in V} {}^2D^1_{a,w} {}^1T_{a,i} Y^{1,*}_{a,\gamma} \quad (3r_D r_T N_o N_v) \quad (3107)$$

$$\tau^6_{\gamma,\alpha,w} = \sum_{i \in O} W^3_{i,\alpha} \tau^5_{\gamma,w,i} \quad (2r_D r_T r_V N_o) \quad (3108)$$

$$\tau^7_{\gamma,w,i} = \sum_{\alpha \in B} W^4_{i,\alpha} \tau^4_{\gamma,\alpha,w} \tau^6_{\gamma,\alpha,w} \quad (3r_D r_T r_V N_o) \quad (3109)$$

$${}^2R^2_{i,\gamma} \leftarrow - \sum_{w \in D} {}^2D^2_{i,w} \tau^7_{\gamma,w,i} \quad (2r_D r_T N_o) \quad (3110)$$

Raw expression

$${}^2R^2_{i,\epsilon} \leftarrow \sum_{\gamma \in A} \sum_{j \in O} \sum_{a \in V} \sum_{b \in V} \sum_{c \in V} \sum_{d \in V} {}^1T_{c,i} {}^1T_{d,j} Y^{1,*}_{a,\epsilon} Z^*_{\epsilon,\gamma} Y^{3,*}_{b,\gamma} Y^{4,*}_{j,\gamma} {}^2D^{a,i,b,j}_{a,c,b,d} V_{a,c,b,d} \quad (3111)$$

Factorized expression

$$\tau^0_{\gamma,\alpha,w} = \sum_{a \in V} {}^2D^1_{a,w} W^1_{a,\alpha} Y^{1,*}_{a,\gamma} \quad (3r_D r_T r_V N_v) \quad (3112)$$

$$\tau^1_{\gamma,w,i} = \sum_{a \in V} {}^2D^3_{a,w} {}^1T_{a,i} Y^{3,*}_{a,\gamma} \quad (3r_D r_T N_o N_v) \quad (3113)$$

$$\tau^2_{\gamma,\alpha,w} = \sum_{i \in O} W^3_{i,\alpha} \tau^1_{\gamma,w,i} \quad (2r_D r_T r_V N_o) \quad (3114)$$

$$\tau^3_{\gamma,\alpha,w} = \sum_{i \in O} {}^2D^4_{i,w} W^4_{i,\alpha} Y^{4,*}_{i,\gamma} \quad (3r_D r_T r_V N_o) \quad (3115)$$

$$\tau^4_{\gamma,\alpha,w} = \sum_{\beta \in B} X_{\alpha,\beta} \tau^2_{\gamma,\beta,w} \tau^3_{\gamma,\beta,w} \quad (3r_D r_T r_V^2) \quad (3116)$$

$$\tau^5_{\gamma,\alpha,w} = \sum_{\delta \in A} Z^*_{\gamma,\delta} \tau^4_{\delta,\alpha,w} \quad (2r_D r_T^2 r_V) \quad (3117)$$

$$\tau^6_{\alpha,i} = \sum_{a \in V} {}^1T_{a,i} W^2_{a,\alpha} \quad (2r_V N_o N_v) \quad (3118)$$

### D. Contributions from $(H^2T)_c$

$$\tau_{\gamma,w,i}^7 = \sum_{\alpha \in B} \tau_{\alpha,i}^6 \tau_{\gamma,\alpha,w}^0 \tau_{\gamma,\alpha,w}^5 \quad (3r_D r_T r_V N_o) \quad (3119)$$

$${}^2R_{i,\gamma}^2 \leftarrow - \sum_{w \in D} {}^2D_{i,w}^2 \tau_{\gamma,w,i}^7 \quad (2r_D r_T N_o) \quad (3120)$$

Raw expression

$${}^2R_{i,\epsilon}^2 \leftarrow \sum_{\gamma \in A} \sum_{j \in O} \sum_{k \in O} \sum_{l \in O} \sum_{a \in V} \sum_{b \in V} {}^1T_{a,k} {}^1T_{b,l} Y_{a,\epsilon}^{1,*} Z_{\epsilon,\gamma}^* Y_{b,\gamma}^{3,*} Y_{j,\gamma}^{4,*} {}^2D_{a,i,b,j} V_{k,i,l,j} \quad (3121)$$

Factorized expression

$$\tau_{\gamma,\alpha,w}^0 = \sum_{a \in V} {}^2D_{a,w}^1 W_{a,\alpha}^1 Y_{a,\gamma}^{1,*} \quad (3r_D r_T r_V N_v) \quad (3122)$$

$$\tau_{\alpha,i}^1 = \sum_{a \in V} {}^1T_{a,i} W_{a,\alpha}^4 \quad (2r_V N_o N_v) \quad (3123)$$

$$\tau_{\gamma,\alpha,w}^2 = \sum_{i \in O} {}^2D_{i,w}^4 Y_{i,\gamma}^{4,*} \tau_{\alpha,i}^1 \quad (3r_D r_T r_V N_o) \quad (3124)$$

$$\tau_{\gamma,w,i}^3 = \sum_{a \in V} {}^2D_{a,w}^3 {}^1T_{a,i} Y_{a,\gamma}^{3,*} \quad (3r_D r_T N_o N_v) \quad (3125)$$

$$\tau_{\gamma,\alpha,w}^4 = \sum_{i \in O} W_{i,\alpha}^3 \tau_{\gamma,w,i}^3 \quad (2r_D r_T r_V N_o) \quad (3126)$$

$$\tau_{\gamma,\alpha,w}^5 = \sum_{\beta \in B} X_{\alpha,\beta} \tau_{\gamma,\beta,w}^2 \tau_{\gamma,\beta,w}^4 \quad (3r_D r_T r_V^2) \quad (3127)$$

$$\tau_{\gamma,\alpha,w}^6 = \sum_{\delta \in A} Z_{\gamma,\delta}^* \tau_{\delta,\alpha,w}^5 \quad (2r_D r_T^2 r_V) \quad (3128)$$

$$\tau_{\gamma,w,i}^7 = \sum_{\alpha \in B} W_{i,\alpha}^2 \tau_{\gamma,\alpha,w}^0 \tau_{\gamma,\alpha,w}^6 \quad (3r_D r_T r_V N_o) \quad (3129)$$

$${}^2R_{i,\gamma}^2 \leftarrow - \sum_{w \in D} {}^2D_{i,w}^2 \tau_{\gamma,w,i}^7 \quad (2r_D r_T N_o) \quad (3130)$$

Raw expression

$${}^2R_{i,\epsilon}^2 \leftarrow \sum_{\gamma \in A} \sum_{j \in O} \sum_{a \in V} \sum_{b \in V} \sum_{c \in V} \frac{1}{2} Y_{a,\epsilon}^{1,*} Z_{\epsilon,\gamma}^* Y_{b,\gamma}^{3,*} Y_{j,\gamma}^{4,*} f_{a,c} {}^2D_{a,i,b,j} {}^2T_{b,j,c,i} \quad (3131)$$

Factorized expression

$$\tau_{\gamma,\alpha}^0 = \sum_{a \in V} W_{a,\alpha}^2 Y_{a,\gamma}^1 \quad (2r_T r_V N_v) \quad (3132)$$

$$\tau_{\gamma,\alpha,a}^1 = \sum_{\beta \in B} W_{a,\beta}^1 X_{\beta,\alpha} \tau_{\gamma,\beta}^0 \quad (3r_T r_V^2 N_v) \quad (3133)$$

$$\tau_{\gamma,\alpha,w}^2 = \sum_{a \in V} {}^2D_{a,w}^3 W_{a,\alpha}^3 Y_{a,\gamma}^{3,*} \quad (3r_D r_T r_V N_v) \quad (3134)$$

$$\tau_{\gamma,\alpha}^3 = \sum_{a \in V} W_{a,\alpha}^4 Y_{a,\gamma}^3 \quad (2r_T r_V N_v) \quad (3135)$$

$$\tau_{\gamma,\alpha,i}^4 = \sum_{\delta \in A} Z_{\gamma,\delta} Y_{i,\delta}^4 \tau_{\delta,\alpha}^3 \quad (3r_T^2 r_V N_o) \quad (3136)$$

$$\tau_{\gamma,\delta,\alpha,w}^5 = \sum_{i \in O} {}^2D_{i,w}^4 Y_{i,\delta}^{4,*} \tau_{\delta,\alpha,w}^2 \tau_{\gamma,\alpha,i}^4 \quad (4r_D r_T^2 r_V N_o) \quad (3137)$$

$$\tau_{\gamma,\delta,w,a}^6 = \sum_{\alpha \in B} \tau_{\gamma,\alpha,a}^1 \tau_{\gamma,\delta,\alpha,w}^5 \quad (2r_D r_T^2 r_V N_v) \quad (3138)$$

$$\tau_{\gamma,i,a}^7 = \sum_{\delta \in A} \sum_{w \in D} {}^2D_{a,w}^1 {}^2D_{i,w}^2 Y_{i,\delta}^2 \tau_{\delta,\gamma,w,a}^6 \quad (4r_D r_T^2 N_o N_v) \quad (3139)$$

$$\tau_{\gamma,\delta,i}^8 = \sum_{a \in V} Y_{a,\gamma}^{1,*} \tau_{\delta,i,a}^7 \quad (2r_T^2 N_o N_v) \quad (3140)$$

$${}^2R_{i,\gamma}^2 \leftarrow \sum_{\delta \in A} \frac{1}{2} Z_{\gamma,\delta}^* \tau_{\gamma,\delta,i}^8 \quad (2r_T^2 N_o) \quad (3141)$$

Raw expression

$${}^2R_{i,\epsilon}^2 \leftarrow \sum_{\gamma \in A} \sum_{j \in O} \sum_{a \in V} \sum_{b \in V} \sum_{c \in V} \frac{1}{2} Y_{a,\epsilon}^{1,*} Z_{\epsilon,\gamma}^* Y_{b,\gamma}^{3,*} Y_{j,\gamma}^{4,*} f_{a,c} {}^2D_{a,i,b,j} {}^2T_{c,i,b,j} \quad (3142)$$

Factorized expression

$$\tau^0_{\gamma,\alpha} = \sum_{a \in V} W^2_{a,\alpha} Y^3_{a,\gamma} \quad (2r_T r_V N_v) \quad (3143)$$

$$\tau^1_{\gamma,\alpha,a} = \sum_{\beta \in B} W^1_{a,\beta} X_{\beta,\alpha} \tau^0_{\gamma,\beta} \quad (3r_T r_V^2 N_v) \quad (3144)$$

$$\tau^2_{\gamma,\alpha,w} = \sum_{a \in V} {}^2D^3_{a,w} W^3_{a,\alpha} Y^{3,*}_{a,\gamma} \quad (3r_D r_T r_V N_v) \quad (3145)$$

$$\tau^3_{\gamma,\alpha} = \sum_{a \in V} W^4_{a,\alpha} Y^1_{a,\gamma} \quad (2r_T r_V N_v) \quad (3146)$$

$$\tau^4_{\gamma,\alpha,i} = \sum_{\delta \in A} Y^2_{i,\delta} Z_{\delta,\gamma} \tau^3_{\delta,\alpha} \quad (3r_T^2 r_V N_o) \quad (3147)$$

$$\tau^5_{\gamma,\delta,\alpha,w} = \sum_{i \in O} {}^2D^4_{i,w} Y^{4,*}_{i,\delta} \tau^2_{\delta,\alpha,w} \tau^4_{\gamma,\alpha,i} \quad (4r_D r_T^2 r_V N_o) \quad (3148)$$

$$\tau^6_{\gamma,\delta,w,a} = \sum_{\alpha \in B} \tau^1_{\gamma,\alpha,a} \tau^5_{\gamma,\delta,\alpha,w} \quad (2r_D r_T^2 r_V N_v) \quad (3149)$$

$$\tau^7_{\gamma,i,a} = \sum_{\delta \in A} \sum_{w \in D} {}^2D^1_{a,w} {}^2D^2_{i,w} Y^4_{i,\delta} \tau^6_{\delta,\gamma,w,a} \quad (4r_D r_T^2 N_o N_v) \quad (3150)$$

$$\tau^8_{\gamma,\delta,i} = \sum_{a \in V} Y^{1,*}_{a,\gamma} \tau^7_{\delta,i,a} \quad (2r_T^2 N_o N_v) \quad (3151)$$

$${}^2R^2_{i,\gamma} \leftarrow \sum_{\delta \in A} \frac{1}{2} Z^*_{\gamma,\delta} \tau^8_{\gamma,\delta,i} \quad (2r_T^2 N_o) \quad (3152)$$

Raw expression

$${}^2R^2_{i,\epsilon} \leftarrow \sum_{\gamma \in A} \sum_{j \in O} \sum_{a \in V} \sum_{b \in V} \sum_{c \in V} \frac{1}{2} Y^{1,*}_{a,\epsilon} Z^*_{\epsilon,\gamma} Y^{3,*}_{b,\gamma} Y^{4,*}_{j,\gamma} f_{b,c} {}^2D^{a,i,b,j} {}^2T_{a,i,c,j} \quad (3153)$$

Factorized expression

$$\tau^0_{\gamma,\delta,w} = \sum_{a \in V} {}^2D^1_{a,w} Y^1_{a,\gamma} Y^{1,*}_{a,\delta} \quad (3r_D r_T^2 N_v) \quad (3154)$$

$$\tau^1_{\gamma,\alpha,w} = \sum_{i \in O} {}^2D^4_{i,w} W^4_{i,\alpha} Y^{4,*}_{i,\gamma} \quad (3r_D r_T r_V N_o) \quad (3155)$$

$$\tau^2_{\gamma,\delta,w} = \sum_{a \in V} {}^2D^3_{a,w} Y^3_{a,\gamma} Y^{3,*}_{a,\delta} \quad (3r_D r_T^2 N_v) \quad (3156)$$

$$\tau^3_{\gamma,\delta,w,i} = \sum_{\epsilon \in A} Z_{\gamma,\epsilon} Y^4_{i,\epsilon} \tau^2_{\epsilon,\delta,w} \quad (3r_D r_T^3 N_o) \quad (3157)$$

$$\tau^4_{\gamma,\delta,\alpha,w} = \sum_{i \in O} W^3_{i,\alpha} \tau^1_{\delta,\alpha,w} \tau^3_{\gamma,\delta,w,i} \quad (3r_D r_T^2 r_V N_o) \quad (3158)$$

$$\tau^5_{\alpha,i,j} = \sum_{\beta \in B} W^1_{i,\beta} W^2_{j,\beta} X_{\beta,\alpha} \quad (3r_V^2 N_o^2) \quad (3159)$$

$$\tau^6_{\gamma,\alpha,i} = \sum_{j \in O} Y^2_{j,\gamma} \tau^5_{\alpha,j,i} \quad (2r_T r_V N_o^2) \quad (3160)$$

$$\tau^7_{\gamma,\delta,w,i} = \sum_{\alpha \in B} \tau^6_{\gamma,\alpha,i} \tau^4_{\gamma,\delta,\alpha,w} \quad (2r_D r_T^2 r_V N_o) \quad (3161)$$

$$\tau^8_{\gamma,\delta,i} = \sum_{\epsilon \in A} \sum_{w \in D} {}^2D^2_{i,w} \tau^0_{\epsilon,\gamma,w} \tau^7_{\epsilon,\delta,w,i} \quad (3r_D r_T^3 N_o) \quad (3162)$$

$${}^2R^2_{i,\gamma} \leftarrow \sum_{\delta \in A} \frac{1}{2} Z^*_{\gamma,\delta} \tau^8_{\gamma,\delta,i} \quad (2r_T^2 N_o) \quad (3163)$$

Raw expression

$${}^2R^2_{i,\epsilon} \leftarrow \sum_{\gamma \in A} \sum_{j \in O} \sum_{a \in V} \sum_{b \in V} \sum_{c \in V} \frac{1}{2} Y^{1,*}_{a,\epsilon} Z^*_{\epsilon,\gamma} Y^{3,*}_{b,\gamma} Y^{4,*}_{j,\gamma} f_{b,c} {}^2D^{a,i,b,j} {}^2T_{c,j,a,i} \quad (3164)$$

Factorized expression

$$\tau^0_{\gamma,\delta,w} = \sum_{a \in V} {}^2D^1_{a,w} Y^3_{a,\gamma} Y^{1,*}_{a,\delta} \quad (3r_D r_T^2 N_v) \quad (3165)$$

$$\tau^1_{\gamma,\alpha,w} = \sum_{i \in O} {}^2D^4_{i,w} W^4_{i,\alpha} Y^{4,*}_{i,\gamma} \quad (3r_D r_T r_V N_o) \quad (3166)$$

$$\tau^2_{\gamma,\delta,w} = \sum_{a \in V} {}^2D^3_{a,w} Y^1_{a,\gamma} Y^{3,*}_{a,\delta} \quad (3r_D r_T^2 N_v) \quad (3167)$$

$$\tau^3_{\gamma,\delta,w,i} = \sum_{\epsilon \in A} Y^2_{i,\epsilon} Z_{\epsilon,\gamma} \tau^2_{\epsilon,\delta,w} \quad (3r_D r_T^3 N_o) \quad (3168)$$

$$\tau^4_{\gamma,\delta,\alpha,w} = \sum_{i \in O} W^3_{i,\alpha} \tau^1_{\delta,\alpha,w} \tau^3_{\gamma,\delta,w,i} \quad (3r_D r_T^2 r_V N_o) \quad (3169)$$

$$\tau^5_{\alpha,i,j} = \sum_{\beta \in B} W^1_{i,\beta} W^2_{j,\beta} X_{\beta,\alpha} \quad (3r_V^2 N_o^2) \quad (3170)$$

$$\tau^6_{\gamma,\alpha,i} = \sum_{j \in O} Y^4_{j,\gamma} \tau^5_{\alpha,j,i} \quad (2r_T r_V N_o^2) \quad (3171)$$

$$\tau^7_{\gamma,\delta,w,i} = \sum_{\alpha \in B} \tau^6_{\gamma,\alpha,i} \tau^4_{\gamma,\delta,\alpha,w} \quad (2r_D r_T^2 r_V N_o) \quad (3172)$$

$$\tau^8_{\gamma,\delta,i} = \sum_{\epsilon \in A} \sum_{w \in D} {}^2D^2_{i,w} \tau^0_{\epsilon,\gamma,w} \tau^7_{\epsilon,\delta,w,i} \quad (3r_D r_T^3 N_o) \quad (3173)$$

$${}^2R^2_{i,\gamma} \leftarrow \sum_{\delta \in A} \frac{1}{2} Z^*_{\gamma,\delta} \tau^8_{\gamma,\delta,i} \quad (2r_T^2 N_o) \quad (3174)$$

Raw expression

$${}^2R^2_{i,\epsilon} \leftarrow \sum_{\gamma \in A} \sum_{j \in O} \sum_{k \in O} \sum_{a \in V} \sum_{b \in V} \sum_{c \in V} Y^{1,*}_{a,\epsilon} Z^*_{\epsilon,\gamma} Y^{3,*}_{b,\gamma} Y^{4,*}_{j,\gamma} {}^2D^{a,i,b,j} {}^2T_{a,i,c,k} V_{b,j,k,c} \quad (3175)$$

Factorized expression

$$\tau^0_{\gamma,\delta,w} = \sum_{a \in V} {}^2D^3_{a,w} Y^3_{a,\gamma} Y^{3,*}_{a,\delta} \quad (3r_D r_T^2 N_v) \quad (3176)$$

$$\tau^1_{\gamma,i} = \sum_{j \in O} Y^4_{j,\gamma} f_{j,i} \quad (2r_T N_o^2) \quad (3177)$$

$$\tau^2_{\gamma,\delta,w} = \sum_{i \in O} {}^2D^4_{i,w} Y^{4,*}_{i,\delta} \tau^1_{\gamma,i} \quad (3r_D r_T^2 N_o) \quad (3178)$$

$$\tau^3_{\gamma,\delta,w} = \sum_{\epsilon \in A} Z^*_{\delta,\epsilon} \tau^0_{\gamma,\epsilon,w} \tau^2_{\gamma,\epsilon,w} \quad (3r_D r_T^3) \quad (3179)$$

$$\tau^4_{\gamma,\delta,w} = \sum_{\epsilon \in A} Z_{\gamma,\epsilon} \tau^3_{\epsilon,\delta,w} \quad (2r_D r_T^3) \quad (3180)$$

$$\tau^5_{\gamma,\delta,w} = \sum_{a \in V} {}^2D^1_{a,w} Y^1_{a,\gamma} Y^{1,*}_{a,\delta} \quad (3r_D r_T^2 N_v) \quad (3181)$$

$${}^2R^2_{i,\gamma} \leftarrow - \sum_{\delta \in A} \sum_{w \in D} \frac{1}{2} {}^2D^2_{i,w} Y^2_{i,\delta} \tau^4_{\delta,\gamma,w} \tau^5_{\delta,\gamma,w} \quad (4r_D r_T^2 N_o) \quad (3182)$$

Raw expression

$${}^2R^2_{i,\epsilon} \leftarrow \sum_{\gamma \in A} \sum_{j \in O} \sum_{k \in O} \sum_{a \in V} \sum_{b \in V} \sum_{c \in V} Y^{1,*}_{a,\epsilon} Z^*_{\epsilon,\gamma} Y^{3,*}_{b,\gamma} Y^{4,*}_{j,\gamma} {}^2D^{a,i,b,j} {}^2T_{b,j,c,k} V_{a,i,k,c} \quad (3183)$$

Factorized expression

$$\tau^0_{\gamma,\delta,w} = \sum_{a \in V} {}^2D^1_{a,w} Y^1_{a,\gamma} Y^{1,*}_{a,\delta} \quad (3r_D r_T^2 N_v) \quad (3184)$$

$$\tau^1_{\gamma,\delta,w} = \sum_{a \in V} {}^2D^3_{a,w} Y^3_{a,\gamma} Y^{3,*}_{a,\delta} \quad (3r_D r_T^2 N_v) \quad (3185)$$

$$\tau^2_{\gamma,\delta,w} = \sum_{i \in O} {}^2D^4_{i,w} Y^4_{i,\gamma} Y^{4,*}_{i,\delta} \quad (3r_D r_T^2 N_o) \quad (3186)$$

$$\tau^3_{\gamma,\delta,w} = \sum_{\epsilon \in A} Z^*_{\delta,\epsilon} \tau^1_{\gamma,\epsilon,w} \tau^2_{\gamma,\epsilon,w} \quad (3r_D r_T^3) \quad (3187)$$

$$\tau^4_{\gamma,\delta,w} = \sum_{\epsilon \in A} Z_{\gamma,\epsilon} \tau^3_{\epsilon,\delta,w} \quad (2r_D r_T^3) \quad (3188)$$

$$\tau^5_{\gamma,i} = \sum_{j \in O} Y^2_{j,\gamma} f_{j,i} \quad (2r_T N_o^2) \quad (3189)$$

$${}^2R^2_{i,\gamma} \leftarrow - \sum_{\delta \in A} \sum_{w \in D} \frac{1}{2} {}^2D^2_{i,w} \tau^5_{\delta,i} \tau^0_{\delta,\gamma,w} \tau^4_{\delta,\gamma,w} \quad (4r_D r_T^2 N_o) \quad (3190)$$

Raw expression

$${}^2R^2_{i,\epsilon} \leftarrow \sum_{\gamma \in A} \sum_{j \in O} \sum_{k \in O} \sum_{a \in V} \sum_{b \in V} \sum_{c \in V} Y^{1,*}_{a,\epsilon} Z^*_{\epsilon,\gamma} Y^{3,*}_{b,\gamma} Y^{4,*}_{j,\gamma} {}^2D^{a,i,b,j} {}^2T_{c,k,a,i} V_{b,j,k,c} \quad (3191)$$

Factorized expression

$$\tau^0_{\gamma,\delta,w} = \sum_{a \in V} {}^2D^3_{a,w} Y^1_{a,\gamma} Y^{3,*}_{a,\delta} \quad (3r_D r_T^2 N_v) \quad (3192)$$

$$\tau^1_{\gamma,\delta,w} = \sum_{i \in O} {}^2D^4_{i,w} Y^2_{i,\gamma} Y^{4,*}_{i,\delta} \quad (3r_D r_T^2 N_o) \quad (3193)$$

$$\tau_{\gamma,\delta,w}^2 = \sum_{\epsilon \in A} Z_{\delta,\epsilon}^* \tau_{\gamma,\epsilon,w}^0 \tau_{\gamma,\epsilon,w}^1 \quad (3r_D r_T^3) \quad (3194)$$

$$\tau_{\gamma,\delta,w}^3 = \sum_{\epsilon \in A} Z_{\epsilon,\gamma} \tau_{\epsilon,\delta,w}^2 \quad (2r_D r_T^3) \quad (3195)$$

$$\tau_{\gamma,\delta,w}^4 = \sum_{a \in V} {}^2D_{a,w}^1 Y_{a,\gamma}^3 Y_{a,\delta}^{1,*} \quad (3r_D r_T^2 N_v) \quad (3196)$$

$$\tau_{\gamma,i}^5 = \sum_{j \in O} Y_{j,\gamma}^4 f_{j,i} \quad (2r_T N_o^2) \quad (3197)$$

$${}^2R_{i,\gamma}^2 \leftarrow - \sum_{\delta \in A} \sum_{w \in D} \frac{1}{2} {}^2D_{i,w}^2 \tau_{\delta,i}^5 \tau_{\delta,\gamma,w}^3 \tau_{\delta,\gamma,w}^4 \quad (4r_D r_T^2 N_o) \quad (3198)$$

Raw expression

$${}^2R_{i,\epsilon}^2 \leftarrow \sum_{\gamma \in A} \sum_{j \in O} \sum_{k \in O} \sum_{a \in V} \sum_{b \in V} \sum_{c \in V} Y_{a,\epsilon}^{1,*} Z_{\epsilon,\gamma}^* Y_{b,\gamma}^{3,*} Y_{j,\gamma}^{4,*} {}^2D_{a,i,b,j} {}^2T_{c,k,b,j} V_{a,i,k,c} \quad (3199)$$

Factorized expression

$$\tau_{\gamma,\delta,w}^0 = \sum_{a \in V} {}^2D_{a,w}^3 Y_{a,\gamma}^1 Y_{a,\delta}^{3,*} \quad (3r_D r_T^2 N_v) \quad (3200)$$

$$\tau_{\gamma,i}^1 = \sum_{j \in O} Y_{j,\gamma}^2 f_{j,i} \quad (2r_T N_o^2) \quad (3201)$$

$$\tau_{\gamma,\delta,w}^2 = \sum_{i \in O} {}^2D_{i,w}^4 Y_{i,\delta}^{4,*} \tau_{\gamma,i}^1 \quad (3r_D r_T^2 N_o) \quad (3202)$$

$$\tau_{\gamma,\delta,w}^3 = \sum_{\epsilon \in A} Z_{\delta,\epsilon}^* \tau_{\gamma,\epsilon,w}^0 \tau_{\gamma,\epsilon,w}^2 \quad (3r_D r_T^3) \quad (3203)$$

$$\tau_{\gamma,\delta,w}^4 = \sum_{\epsilon \in A} Z_{\epsilon,\gamma} \tau_{\epsilon,\delta,w}^3 \quad (2r_D r_T^3) \quad (3204)$$

$$\tau_{\gamma,\delta,w}^5 = \sum_{a \in V} {}^2D_{a,w}^1 Y_{a,\gamma}^3 Y_{a,\delta}^{1,*} \quad (3r_D r_T^2 N_v) \quad (3205)$$

$${}^2R_{i,\gamma}^2 \leftarrow - \sum_{\delta \in A} \sum_{w \in D} \frac{1}{2} {}^2D_{i,w}^2 Y_{i,\delta}^4 \tau_{\delta,\gamma,w}^4 \tau_{\delta,\gamma,w}^5 \quad (4r_D r_T^2 N_o) \quad (3206)$$

Raw expression

$${}^2R_{i,\epsilon}^2 \leftarrow - \sum_{\gamma \in A} \sum_{j \in O} \sum_{k \in O} \sum_{a \in V} \sum_{b \in V} \sum_{c \in V} \frac{1}{2} Y_{a,\epsilon}^{1,*} Z_{\epsilon,\gamma}^* Y_{b,\gamma}^{3,*} Y_{j,\gamma}^{4,*} {}^2D_{a,i,b,j} {}^2T_{a,i,c,k} V_{b,c,k,j} \quad (3207)$$

Factorized expression

$$\tau_{\gamma,\delta,w}^0 = \sum_{a \in V} {}^2D_{a,w}^1 Y_{a,\gamma}^1 Y_{a,\delta}^{1,*} \quad (3r_D r_T^2 N_v) \quad (3208)$$

$$\tau_{\gamma,\delta,w}^1 = \sum_{i \in O} {}^2D_{i,w}^4 Y_{i,\gamma}^4 Y_{i,\delta}^{4,*} \quad (3r_D r_T^2 N_o) \quad (3209)$$

$$\tau_{\gamma,a}^2 = \sum_{b \in V} Y_{b,\gamma}^3 f_{a,b} \quad (2r_T N_v^2) \quad (3210)$$

$$\tau_{\gamma,\delta,w}^3 = \sum_{a \in V} {}^2D_{a,w}^3 Y_{a,\delta}^{3,*} \tau_{\gamma,a}^2 \quad (3r_D r_T^2 N_v) \quad (3211)$$

$$\tau_{\gamma,\delta,w}^4 = \sum_{\epsilon \in A} Z_{\delta,\epsilon}^* \tau_{\gamma,\epsilon,w}^1 \tau_{\gamma,\epsilon,w}^3 \quad (3r_D r_T^3) \quad (3212)$$

$$\tau_{\gamma,\delta,w}^5 = \sum_{\epsilon \in A} Z_{\gamma,\epsilon} \tau_{\epsilon,\delta,w}^4 \quad (2r_D r_T^3) \quad (3213)$$

$${}^2R_{i,\gamma}^2 \leftarrow \sum_{\delta \in A} \sum_{w \in D} \frac{1}{2} {}^2D_{i,w}^2 Y_{i,\delta}^2 \tau_{\delta,\gamma,w}^0 \tau_{\delta,\gamma,w}^5 \quad (4r_D r_T^2 N_o) \quad (3214)$$

Raw expression

$${}^2R_{i,\epsilon}^2 \leftarrow - \sum_{\gamma \in A} \sum_{j \in O} \sum_{k \in O} \sum_{a \in V} \sum_{b \in V} \sum_{c \in V} \frac{1}{2} Y_{a,\epsilon}^{1,*} Z_{\epsilon,\gamma}^* Y_{b,\gamma}^{3,*} Y_{j,\gamma}^{4,*} {}^2D_{a,i,b,j} {}^2T_{a,k,c,i} V_{b,j,k,c} \quad (3215)$$

Factorized expression

$$\tau_{\gamma,a}^0 = \sum_{b \in V} Y_{b,\gamma}^3 f_{a,b} \quad (2r_T N_v^2) \quad (3216)$$

$$\tau_{\gamma,\delta,w}^1 = \sum_{a \in V} {}^2D_{a,w}^1 Y_{a,\gamma}^{1,*} \tau_{\gamma,a}^0 \quad (3r_D r_T^2 N_v) \quad (3217)$$

$$\tau_{\gamma,\delta,w}^2 = \sum_{a \in V} {}^2D_{a,w}^3 Y_{a,\gamma}^1 Y_{a,\delta}^{3,*} \quad (3r_D r_T^2 N_v) \quad (3218)$$

$$\tau^3_{\gamma,\delta,w} = \sum_{i \in O} {}^2D^4_{i,w} Y^2_{i,\gamma} Y^{4,*}_{i,\delta} \quad (3r_D r_T^2 N_o) \quad (3219)$$

$$\tau^4_{\gamma,\delta,w} = \sum_{\epsilon \in A} Z^*_{\delta,\epsilon} \tau^2_{\gamma,\epsilon,w} \tau^3_{\gamma,\epsilon,w} \quad (3r_D r_T^3) \quad (3220)$$

$$\tau^5_{\gamma,\delta,w} = \sum_{\epsilon \in A} Z_{\epsilon,\gamma} \tau^4_{\epsilon,\delta,w} \quad (2r_D r_T^3) \quad (3221)$$

$${}^2R^2_{i,\gamma} \leftarrow \sum_{\delta \in A} \sum_{w \in D} \frac{1}{2} {}^2D^2_{i,w} Y^4_{i,\delta} \tau^1_{\delta,\gamma,w} \tau^5_{\delta,\gamma,w} \quad (4r_D r_T^2 N_o) \quad (3222)$$

Raw expression

$${}^2R^2_{i,\epsilon} \leftarrow - \sum_{\gamma \in A} \sum_{j \in O} \sum_{k \in O} \sum_{a \in V} \sum_{b \in V} \sum_{c \in V} \frac{1}{2} Y^{1,*}_{a,\epsilon} Z^*_{\epsilon,\gamma} Y^{3,*}_{b,\gamma} Y^{4,*}_{j,\gamma} {}^2D^{a,i,b,j} {}^2T_{a,k,c,j} V_{b,c,k,i} \quad (3223)$$

Factorized expression

$$\tau^0_{\gamma,a} = \sum_{b \in V} Y^1_{b,\gamma} f_{a,b} \quad (2r_T N_v^2) \quad (3224)$$

$$\tau^1_{\gamma,\delta,w} = \sum_{a \in V} {}^2D^1_{a,w} Y^{1,*}_{a,\delta} \tau^0_{\gamma,a} \quad (3r_D r_T^2 N_v) \quad (3225)$$

$$\tau^2_{\gamma,\delta,w} = \sum_{a \in V} {}^2D^3_{a,w} Y^3_{a,\gamma} Y^{3,*}_{a,\delta} \quad (3r_D r_T^2 N_v) \quad (3226)$$

$$\tau^3_{\gamma,\delta,w} = \sum_{i \in O} {}^2D^4_{i,w} Y^4_{i,\gamma} Y^{4,*}_{i,\delta} \quad (3r_D r_T^2 N_o) \quad (3227)$$

$$\tau^4_{\gamma,\delta,w} = \sum_{\epsilon \in A} Z^*_{\delta,\epsilon} \tau^2_{\gamma,\epsilon,w} \tau^3_{\gamma,\epsilon,w} \quad (3r_D r_T^3) \quad (3228)$$

$$\tau^5_{\gamma,\delta,w} = \sum_{\epsilon \in A} Z_{\gamma,\epsilon} \tau^4_{\epsilon,\delta,w} \quad (2r_D r_T^3) \quad (3229)$$

$${}^2R^2_{i,\gamma} \leftarrow \sum_{\delta \in A} \sum_{w \in D} \frac{1}{2} {}^2D^2_{i,w} Y^2_{i,\delta} \tau^1_{\delta,\gamma,w} \tau^5_{\delta,\gamma,w} \quad (4r_D r_T^2 N_o) \quad (3230)$$

Raw expression

$${}^2R^2_{i,\epsilon} \leftarrow - \sum_{\gamma \in A} \sum_{j \in O} \sum_{k \in O} \sum_{a \in V} \sum_{b \in V} \sum_{c \in V} \frac{1}{2} Y^{1,*}_{a,\epsilon} Z^*_{\epsilon,\gamma} Y^{3,*}_{b,\gamma} Y^{4,*}_{j,\gamma} {}^2D^{a,i,b,j} {}^2T_{b,j,c,k} V_{a,c,k,i} \quad (3231)$$

Factorized expression

$$\tau^0_{\gamma,\delta,w} = \sum_{i \in O} {}^2D^4_{i,w} Y^2_{i,\gamma} Y^{4,*}_{i,\delta} \quad (3r_D r_T^2 N_o) \quad (3232)$$

$$\tau^1_{\gamma,a} = \sum_{b \in V} Y^1_{b,\gamma} f_{a,b} \quad (2r_T N_v^2) \quad (3233)$$

$$\tau^2_{\gamma,\delta,w} = \sum_{a \in V} {}^2D^3_{a,w} Y^{3,*}_{a,\delta} \tau^1_{\gamma,a} \quad (3r_D r_T^2 N_v) \quad (3234)$$

$$\tau^3_{\gamma,\delta,w} = \sum_{\epsilon \in A} Z^*_{\delta,\epsilon} \tau^0_{\gamma,\epsilon,w} \tau^2_{\gamma,\epsilon,w} \quad (3r_D r_T^3) \quad (3235)$$

$$\tau^4_{\gamma,\delta,w} = \sum_{\epsilon \in A} Z_{\epsilon,\gamma} \tau^3_{\epsilon,\delta,w} \quad (2r_D r_T^3) \quad (3236)$$

$$\tau^5_{\gamma,\delta,w} = \sum_{a \in V} {}^2D^1_{a,w} Y^3_{a,\gamma} Y^{1,*}_{a,\delta} \quad (3r_D r_T^2 N_v) \quad (3237)$$

$${}^2R^2_{i,\gamma} \leftarrow \sum_{\delta \in A} \sum_{w \in D} \frac{1}{2} {}^2D^2_{i,w} Y^4_{i,\delta} \tau^4_{\delta,\gamma,w} \tau^5_{\delta,\gamma,w} \quad (4r_D r_T^2 N_o) \quad (3238)$$

Raw expression

$${}^2R^2_{i,\epsilon} \leftarrow - \sum_{\gamma \in A} \sum_{j \in O} \sum_{k \in O} \sum_{a \in V} \sum_{b \in V} \sum_{c \in V} \frac{1}{2} Y^{1,*}_{a,\epsilon} Z^*_{\epsilon,\gamma} Y^{3,*}_{b,\gamma} Y^{4,*}_{j,\gamma} {}^2D^{a,i,b,j} {}^2T_{b,k,c,i} V_{a,c,k,j} \quad (3239)$$

Factorized expression

$$\tau^0_{\gamma,\alpha,w} = \sum_{a \in V} {}^2D^1_{a,w} W^1_{a,\alpha} Y^{1,*}_{a,\gamma} \quad (3r_D r_T r_V N_v) \quad (3240)$$

$$\tau^1_{\gamma,\alpha} = \sum_{a \in V} W^4_{a,\alpha} Y^3_{a,\gamma} \quad (2r_T r_V N_v) \quad (3241)$$

$$\tau^2_{\gamma,\alpha} = \sum_{i \in O} W^3_{i,\alpha} Y^4_{i,\gamma} \quad (2r_T r_V N_o) \quad (3242)$$



$$\tau^3_{\gamma,\alpha} = \sum_{\beta \in B} X_{\alpha,\beta} \tau^1_{\gamma,\beta} \tau^2_{\gamma,\beta} \quad (3r_T r_V^2) \quad (3243)$$

$$\tau^4_{\gamma,\alpha} = \sum_{\delta \in A} Z_{\gamma,\delta} \tau^3_{\delta,\alpha} \quad (2r_T^2 r_V) \quad (3244)$$

$$\tau^5_{\gamma,\delta,w} = \sum_{a \in V} {}^2D^3_{a,w} Y^1_{a,\gamma} Y^{3,*}_{a,\delta} \quad (3r_D r_T^2 N_v) \quad (3245)$$

$$\tau^6_{\gamma,\delta,w} = \sum_{i \in O} {}^2D^4_{i,w} Y^2_{i,\gamma} Y^{4,*}_{i,\delta} \quad (3r_D r_T^2 N_o) \quad (3246)$$

$$\tau^7_{\gamma,\delta,w} = \sum_{\epsilon \in A} Z^*_{\delta,\epsilon} \tau^5_{\gamma,\epsilon,w} \tau^6_{\gamma,\epsilon,w} \quad (3r_D r_T^3) \quad (3247)$$

$$\tau^8_{\gamma,\alpha,w} = \sum_{\delta \in A} \tau^4_{\delta,\alpha} \tau^7_{\delta,\gamma,w} \quad (2r_D r_T^2 r_V) \quad (3248)$$

$$\tau^9_{\gamma,w,i} = \sum_{\alpha \in B} W^2_{i,\alpha} \tau^0_{\gamma,\alpha,w} \tau^8_{\gamma,\alpha,w} \quad (3r_D r_T r_V N_o) \quad (3249)$$

$${}^2R^2_{i,\gamma} \leftarrow \sum_{w \in D} {}^2D^2_{i,w} \tau^9_{\gamma,w,i} \quad (2r_D r_T N_o) \quad (3250)$$

Raw expression

$${}^2R^2_{i,\epsilon} \leftarrow - \sum_{\gamma \in A} \sum_{j \in O} \sum_{k \in O} \sum_{a \in V} \sum_{b \in V} \sum_{c \in V} \frac{1}{2} Y^{1,*}_{a,\epsilon} Z^*_{\epsilon,\gamma} Y^{3,*}_{b,\gamma} Y^{4,*}_{j,\gamma} {}^2D^{a,i,b,j} {}^2T_{b,k,c,j} V_{a,i,k,c} \quad (3251)$$

Factorized expression

$$\tau^0_{\gamma,\alpha,w} = \sum_{a \in V} {}^2D^1_{a,w} W^1_{a,\alpha} Y^{1,*}_{a,\gamma} \quad (3r_D r_T r_V N_v) \quad (3252)$$

$$\tau^1_{\gamma,\delta,w} = \sum_{a \in V} {}^2D^3_{a,w} Y^3_{a,\gamma} Y^{3,*}_{a,\delta} \quad (3r_D r_T^2 N_v) \quad (3253)$$

$$\tau^2_{\gamma,\delta,w} = \sum_{i \in O} {}^2D^4_{i,w} Y^4_{i,\gamma} Y^{4,*}_{i,\delta} \quad (3r_D r_T^2 N_o) \quad (3254)$$

$$\tau^3_{\gamma,\delta,w} = \sum_{\epsilon \in A} Z^*_{\delta,\epsilon} \tau^1_{\gamma,\epsilon,w} \tau^2_{\gamma,\epsilon,w} \quad (3r_D r_T^3) \quad (3255)$$

$$\tau^4_{\gamma,\alpha} = \sum_{a \in V} W^4_{a,\alpha} Y^1_{a,\gamma} \quad (2r_T r_V N_v) \quad (3256)$$

$$\tau^5_{\gamma,\alpha} = \sum_{i \in O} W^3_{i,\alpha} Y^2_{i,\gamma} \quad (2r_T r_V N_o) \quad (3257)$$

$$\tau^6_{\gamma,\alpha} = \sum_{\beta \in B} X_{\alpha,\beta} \tau^4_{\gamma,\beta} \tau^5_{\gamma,\beta} \quad (3r_T r_V^2) \quad (3258)$$

$$\tau^7_{\gamma,\alpha} = \sum_{\delta \in A} Z_{\delta,\gamma} \tau^6_{\delta,\alpha} \quad (2r_T^2 r_V) \quad (3259)$$

$$\tau^8_{\gamma,\alpha,w} = \sum_{\delta \in A} \tau^7_{\delta,\alpha} \tau^3_{\delta,\gamma,w} \quad (2r_D r_T^2 r_V) \quad (3260)$$

$$\tau^9_{\gamma,w,i} = \sum_{\alpha \in B} W^2_{i,\alpha} \tau^0_{\gamma,\alpha,w} \tau^8_{\gamma,\alpha,w} \quad (3r_D r_T r_V N_o) \quad (3261)$$

$${}^2R^2_{i,\gamma} \leftarrow \sum_{w \in D} {}^2D^2_{i,w} \tau^9_{\gamma,w,i} \quad (2r_D r_T N_o) \quad (3262)$$

Raw expression

$${}^2R^2_{i,\epsilon} \leftarrow - \sum_{\gamma \in A} \sum_{j \in O} \sum_{k \in O} \sum_{a \in V} \sum_{b \in V} \sum_{c \in V} \frac{1}{2} Y^{1,*}_{a,\epsilon} Z^*_{\epsilon,\gamma} Y^{3,*}_{b,\gamma} Y^{4,*}_{j,\gamma} {}^2D^{a,i,b,j} {}^2T_{c,i,a,k} V_{b,j,k,c} \quad (3263)$$

Factorized expression

$$\tau^0_{\gamma,\delta,w} = \sum_{a \in V} {}^2D^1_{a,w} Y^1_{a,\gamma} Y^{1,*}_{a,\delta} \quad (3r_D r_T^2 N_v) \quad (3264)$$

$$\tau^1_{\gamma,\alpha,w} = \sum_{a \in V} {}^2D^3_{a,w} W^1_{a,\alpha} Y^{3,*}_{a,\gamma} \quad (3r_D r_T r_V N_v) \quad (3265)$$

$$\tau^2_{\gamma,\alpha,w} = \sum_{i \in O} {}^2D^4_{i,w} W^2_{i,\alpha} Y^{4,*}_{i,\gamma} \quad (3r_D r_T r_V N_o) \quad (3266)$$

$$\tau^3_{\gamma,\alpha} = \sum_{a \in V} W^4_{a,\alpha} Y^3_{a,\gamma} \quad (2r_T r_V N_v) \quad (3267)$$

$$\tau^4_{\gamma,\alpha} = \sum_{i \in O} W^3_{i,\alpha} Y^4_{i,\gamma} \quad (2r_T r_V N_o) \quad (3268)$$

$$\tau^5_{\gamma,\alpha} = \sum_{\beta \in B} X_{\alpha,\beta} \tau^3_{\gamma,\beta} \tau^4_{\gamma,\beta} \quad (3r_T r_V^2) \quad (3269)$$

$$\tau^7_{\gamma,\delta,w} = \sum_{\alpha \in B} \tau^6_{\gamma,\alpha} \tau^1_{\delta,\alpha,w} \tau^2_{\delta,\alpha,w} \quad (3r_D r_T^2 r_V) \quad (3282)$$

$$\tau^6_{\gamma,\alpha} = \sum_{\delta \in A} Z_{\gamma,\delta} \tau^5_{\delta,\alpha} \quad (2r_T^2 r_V) \quad (3270)$$

$$\tau^8_{\gamma,\delta,w} = \sum_{\epsilon \in A} Z^*_{\delta,\epsilon} \tau^7_{\gamma,\epsilon,w} \quad (2r_D r_T^3) \quad (3283)$$

$$\tau^7_{\gamma,\delta,w} = \sum_{\alpha \in B} \tau^6_{\gamma,\alpha} \tau^1_{\delta,\alpha,w} \tau^2_{\delta,\alpha,w} \quad (3r_D r_T^2 r_V) \quad (3271)$$

$${}^2R^2_{i,\gamma} \leftarrow \sum_{\delta \in A} \sum_{w \in D} {}^2D^2_{i,w} Y^4_{i,\delta} \tau^0_{\delta,\gamma,w} \tau^8_{\delta,\gamma,w} \quad (4r_D r_T^2 N_o) \quad (3284)$$

$$\tau^8_{\gamma,\delta,w} = \sum_{\epsilon \in A} Z^*_{\delta,\epsilon} \tau^7_{\gamma,\epsilon,w} \quad (2r_D r_T^3) \quad (3272)$$

Raw expression

$${}^2R^2_{i,\gamma} \leftarrow \sum_{\delta \in A} \sum_{w \in D} {}^2D^2_{i,w} Y^2_{i,\delta} \tau^0_{\delta,\gamma,w} \tau^8_{\delta,\gamma,w} \quad (4r_D r_T^2 N_o) \quad (3273)$$

$${}^2R^2_{i,\epsilon} \leftarrow - \sum_{\gamma \in A} \sum_{j \in O} \sum_{k \in O} \sum_{a \in V} \sum_{b \in V} \sum_{c \in V} \frac{1}{2} Y^{1,*}_{a,\epsilon} Z^*_{\epsilon,\gamma} Y^{3,*}_{b,\gamma} Y^{4,*}_{j,\gamma} {}^2D^{a,i,b,j} {}^2T_{c,j,a,k} V_{b,c,k,i} \quad (3285)$$

Raw expression

$${}^2R^2_{i,\epsilon} \leftarrow - \sum_{\gamma \in A} \sum_{j \in O} \sum_{k \in O} \sum_{a \in V} \sum_{b \in V} \sum_{c \in V} \frac{1}{2} Y^{1,*}_{a,\epsilon} Z^*_{\epsilon,\gamma} Y^{3,*}_{b,\gamma} Y^{4,*}_{j,\gamma} {}^2D^{a,i,b,j} {}^2T_{c,i,b,k} V_{a,c,k,j} \quad (3274)$$

Factorized expression

$$\tau^0_{\alpha,i,j} = \sum_{\beta \in B} X_{\alpha,\beta} W^3_{i,\beta} W^4_{j,\beta} \quad (3r_V^2 N_o^2) \quad (3286)$$

Factorized expression

$$\tau^1_{\gamma,\alpha,i} = \sum_{j \in O} Y^4_{j,\gamma} \tau^0_{\alpha,j,i} \quad (2r_T r_V N_o^2) \quad (3287)$$

$$\tau^0_{\gamma,\delta,w} = \sum_{a \in V} {}^2D^1_{a,w} Y^3_{a,\gamma} Y^{1,*}_{a,\delta} \quad (3r_D r_T^2 N_v) \quad (3275)$$

$$\tau^2_{\gamma,\alpha} = \sum_{a \in V} W^2_{a,\alpha} Y^3_{a,\gamma} \quad (2r_T r_V N_v) \quad (3288)$$

$$\tau^1_{\gamma,\alpha,w} = \sum_{a \in V} {}^2D^3_{a,w} W^1_{a,\alpha} Y^{3,*}_{a,\gamma} \quad (3r_D r_T r_V N_v) \quad (3276)$$

$$\tau^3_{\gamma,i,a} = \sum_{\alpha \in B} W^1_{a,\alpha} \tau^2_{\gamma,\alpha} \tau^1_{\gamma,\alpha,i} \quad (3r_T r_V N_o N_v) \quad (3289)$$

$$\tau^2_{\gamma,\alpha,w} = \sum_{i \in O} {}^2D^4_{i,w} W^2_{i,\alpha} Y^{4,*}_{i,\gamma} \quad (3r_D r_T r_V N_o) \quad (3277)$$

$$\tau^4_{\gamma,\delta,w} = \sum_{a \in V} {}^2D^3_{a,w} Y^1_{a,\gamma} Y^{3,*}_{a,\delta} \quad (3r_D r_T^2 N_v) \quad (3290)$$

$$\tau^3_{\gamma,\alpha} = \sum_{a \in V} W^4_{a,\alpha} Y^1_{a,\gamma} \quad (2r_T r_V N_v) \quad (3278)$$

$$\tau^5_{\gamma,\delta,w} = \sum_{i \in O} {}^2D^4_{i,w} Y^2_{i,\gamma} Y^{4,*}_{i,\delta} \quad (3r_D r_T^2 N_o) \quad (3291)$$

$$\tau^4_{\gamma,\alpha} = \sum_{i \in O} W^3_{i,\alpha} Y^2_{i,\gamma} \quad (2r_T r_V N_o) \quad (3279)$$

$$\tau^6_{\gamma,\delta,w} = \sum_{\epsilon \in A} Z^*_{\delta,\epsilon} \tau^4_{\gamma,\epsilon,w} \tau^5_{\gamma,\epsilon,w} \quad (3r_D r_T^3) \quad (3292)$$

$$\tau^5_{\gamma,\alpha} = \sum_{\beta \in B} X_{\alpha,\beta} \tau^3_{\gamma,\beta} \tau^4_{\gamma,\beta} \quad (3r_T r_V^2) \quad (3280)$$

$$\tau^7_{\gamma,\delta,w} = \sum_{\epsilon \in A} Z_{\epsilon,\gamma} \tau^6_{\epsilon,\delta,w} \quad (2r_D r_T^3) \quad (3293)$$

$$\tau^6_{\gamma,\alpha} = \sum_{\delta \in A} Z_{\delta,\gamma} \tau^5_{\delta,\alpha} \quad (2r_T^2 r_V) \quad (3281)$$

$$\tau^8_{\gamma,i,a} = \sum_{\delta \in A} \sum_{w \in D} {}^2D^1_{a,w} {}^2D^2_{i,w} \tau^3_{\delta,i,a} \tau^7_{\delta,\gamma,w} \quad (4r_D r_T^2 N_o N_v) \quad (3294)$$

$${}^2R^2_{i,\gamma} \leftarrow - \sum_{a \in V} \frac{1}{2} Y^{1,*}_{a,\gamma} \tau^8_{\gamma,i,a} \quad (2r_T N_o N_v) \quad (3295)$$

Raw expression

$${}^2R^2_{i,\epsilon} \leftarrow - \sum_{\gamma \in A} \sum_{j \in O} \sum_{k \in O} \sum_{a \in V} \sum_{b \in V} \sum_{c \in V} \frac{1}{2} Y^{1,*}_{a,\epsilon} Z^*_{\epsilon,\gamma} Y^{3,*}_{b,\gamma} Y^{4,*}_{j,\gamma} {}^2D^{a,i,b,j} {}^2T_{c,j,b,k} V_{a,i,k,c} \quad (3296)$$

Factorized expression

$$\tau^0_{\alpha,i,j} = \sum_{\beta \in B} X_{\alpha,\beta} W^3_{i,\beta} W^4_{j,\beta} \quad (3r_V^2 N_o^2) \quad (3297)$$

$$\tau^1_{\gamma,\alpha,i} = \sum_{j \in O} Y^2_{j,\gamma} \tau^0_{\alpha,j,i} \quad (2r_T r_V N_o^2) \quad (3298)$$

$$\tau^2_{\gamma,\alpha} = \sum_{a \in V} W^2_{a,\alpha} Y^1_{a,\gamma} \quad (2r_T r_V N_v) \quad (3299)$$

$$\tau^3_{\gamma,i,a} = \sum_{\alpha \in B} W^1_{a,\alpha} \tau^2_{\gamma,\alpha} \tau^1_{\gamma,\alpha,i} \quad (3r_T r_V N_o N_v) \quad (3300)$$

$$\tau^4_{\gamma,\delta,w} = \sum_{a \in V} {}^2D^3_{a,w} Y^3_{a,\gamma} Y^{3,*}_{a,\delta} \quad (3r_D r_T^2 N_v) \quad (3301)$$

$$\tau^5_{\gamma,\delta,w} = \sum_{i \in O} {}^2D^4_{i,w} Y^4_{i,\gamma} Y^{4,*}_{i,\delta} \quad (3r_D r_T^2 N_o) \quad (3302)$$

$$\tau^6_{\gamma,\delta,w} = \sum_{\epsilon \in A} Z^*_{\delta,\epsilon} \tau^4_{\gamma,\epsilon,w} \tau^5_{\gamma,\epsilon,w} \quad (3r_D r_T^3) \quad (3303)$$

$$\tau^7_{\gamma,\delta,w} = \sum_{\epsilon \in A} Z_{\gamma,\epsilon} \tau^6_{\epsilon,\delta,w} \quad (2r_D r_T^3) \quad (3304)$$

$$\tau^8_{\gamma,i,a} = \sum_{\delta \in A} \sum_{w \in D} {}^2D^1_{a,w} {}^2D^2_{i,w} \tau^3_{\delta,i,a} \tau^7_{\delta,\gamma,w} \quad (4r_D r_T^2 N_o N_v) \quad (3305)$$

$${}^2R^2_{i,\gamma} \leftarrow - \sum_{a \in V} \frac{1}{2} Y^{1,*}_{a,\gamma} \tau^8_{\gamma,i,a} \quad (2r_T N_o N_v) \quad (3306)$$

Raw expression

$${}^2R^2_{i,\epsilon} \leftarrow - \sum_{\gamma \in A} \sum_{j \in O} \sum_{k \in O} \sum_{a \in V} \sum_{b \in V} \sum_{c \in V} \frac{1}{2} Y^{1,*}_{a,\epsilon} Z^*_{\epsilon,\gamma} Y^{3,*}_{b,\gamma} Y^{4,*}_{j,\gamma} {}^2D^{a,i,b,j} {}^2T_{c,k,a,i} V_{b,c,k,j} \quad (3307)$$

Factorized expression

$$\tau^0_{\gamma,\alpha,w} = \sum_{a \in V} {}^2D^1_{a,w} W^1_{a,\alpha} Y^{1,*}_{a,\gamma} \quad (3r_D r_T r_V N_v) \quad (3308)$$

$$\tau^1_{\gamma,\alpha} = \sum_{a \in V} W^2_{a,\alpha} Y^3_{a,\gamma} \quad (2r_T r_V N_v) \quad (3309)$$

$$\tau^2_{\gamma,\alpha,i} = \sum_{\delta \in A} Z_{\gamma,\delta} Y^4_{i,\delta} \tau^1_{\delta,\alpha} \quad (3r_T^2 r_V N_o) \quad (3310)$$

$$\tau^3_{\gamma,\delta,w} = \sum_{a \in V} {}^2D^3_{a,w} Y^1_{a,\gamma} Y^{3,*}_{a,\delta} \quad (3r_D r_T^2 N_v) \quad (3311)$$

$$\tau^4_{\gamma,\delta,w,i} = \sum_{\epsilon \in A} {}^2D^4_{i,w} Z^*_{\delta,\epsilon} Y^{4,*}_{i,\epsilon} \tau^3_{\gamma,\epsilon,w} \quad (4r_D r_T^3 N_o) \quad (3312)$$

$$\tau^5_{\alpha,i,j} = \sum_{\beta \in B} X_{\alpha,\beta} W^3_{i,\beta} W^4_{j,\beta} \quad (3r_V^2 N_o^2) \quad (3313)$$

$$\tau^6_{\gamma,\alpha,i} = \sum_{j \in O} Y^2_{j,\gamma} \tau^5_{\alpha,j,i} \quad (2r_T r_V N_o^2) \quad (3314)$$

$$\tau^7_{\gamma,\delta,\alpha,w} = \sum_{i \in O} \tau^6_{\gamma,\alpha,i} \tau^4_{\gamma,\delta,w,i} \quad (2r_D r_T^2 r_V N_o) \quad (3315)$$

$$\tau^8_{\gamma,\alpha,w,i} = \sum_{\delta \in A} \tau^2_{\delta,\alpha,i} \tau^7_{\delta,\gamma,\alpha,w} \quad (2r_D r_T^2 r_V N_o) \quad (3316)$$

$$\tau^9_{\gamma,w,i} = \sum_{\alpha \in B} \tau^0_{\gamma,\alpha,w} \tau^8_{\gamma,\alpha,w,i} \quad (2r_D r_T r_V N_o) \quad (3317)$$

$${}^2R^2_{i,\gamma} \leftarrow - \sum_{w \in D} \frac{1}{2} {}^2D^2_{i,w} \tau^9_{\gamma,w,i} \quad (2r_D r_T N_o) \quad (3318)$$

Raw expression

$${}^2R^2_{i,\epsilon} \leftarrow - \sum_{\gamma \in A} \sum_{j \in O} \sum_{k \in O} \sum_{a \in V} \sum_{b \in V} \sum_{c \in V} \frac{1}{2} Y^{1,*}_{a,\epsilon} Z^*_{\epsilon,\gamma} Y^{3,*}_{b,\gamma} Y^{4,*}_{j,\gamma} {}^2D^{a,i,b,j} {}^2T_{c,k,b,j} V_{a,c,k,i} \quad (3319)$$

Factorized expression

$$\tau^0_{\gamma,\alpha,w} = \sum_{a \in V} {}^2D^1_{a,w} W^1_{a,\alpha} Y^{1,*}_{a,\gamma} \quad (3r_D r_T r_V N_v) \quad (3320)$$

$$\tau^1_{\gamma,\delta,w} = \sum_{a \in V} {}^2D^3_{a,w} Y^3_{a,\gamma} Y^{3,*}_{a,\delta} \quad (3r_D r_T^2 N_v) \quad (3321)$$

$$\tau^2_{\gamma,\delta,w,i} = \sum_{\epsilon \in A} {}^2D^4_{i,w} Z^*_{\delta,\epsilon} Y^{4,*}_{i,\epsilon} \tau^1_{\gamma,\epsilon,w} \quad (4r_D r_T^3 N_o) \quad (3322)$$

$$\tau^3_{\alpha,i,j} = \sum_{\beta \in B} X_{\alpha,\beta} W^3_{i,\beta} W^4_{j,\beta} \quad (3r_V^2 N_o^2) \quad (3323)$$

$$\tau^4_{\gamma,\alpha,i} = \sum_{j \in O} Y^4_{j,\gamma} \tau^3_{\alpha,j,i} \quad (2r_T r_V N_o^2) \quad (3324)$$

$$\tau^5_{\gamma,\delta,\alpha,w} = \sum_{i \in O} \tau^4_{\gamma,\alpha,i} \tau^2_{\gamma,\delta,w,i} \quad (2r_D r_T^2 r_V N_o) \quad (3325)$$

$$\tau^6_{\gamma,\alpha} = \sum_{a \in V} W^2_{a,\alpha} Y^1_{a,\gamma} \quad (2r_T r_V N_v) \quad (3326)$$

$$\tau^7_{\gamma,\alpha,i} = \sum_{\delta \in A} Y^2_{i,\delta} Z_{\delta,\gamma} \tau^6_{\delta,\alpha} \quad (3r_T^2 r_V N_o) \quad (3327)$$

$$\tau^8_{\gamma,\alpha,w,i} = \sum_{\delta \in A} \tau^7_{\delta,\alpha,i} \tau^5_{\delta,\gamma,\alpha,w} \quad (2r_D r_T^2 r_V N_o) \quad (3328)$$

$$\tau^9_{\gamma,w,i} = \sum_{\alpha \in B} \tau^0_{\gamma,\alpha,w} \tau^8_{\gamma,\alpha,w,i} \quad (2r_D r_T r_V N_o) \quad (3329)$$

$${}^2R^2_{i,\gamma} \leftarrow - \sum_{w \in D} \frac{1}{2} {}^2D^2_{i,w} \tau^9_{\gamma,w,i} \quad (2r_D r_T N_o) \quad (3330)$$

Raw expression

$${}^2R^2_{i,\epsilon} \leftarrow \sum_{\gamma \in A} \sum_{j \in O} \sum_{a \in V} \sum_{b \in V} \sum_{c \in V} \sum_{d \in V} \frac{1}{2} Y^{1,*}_{a,\epsilon} Z^*_{\epsilon,\gamma} Y^{3,*}_{b,\gamma} Y^{4,*}_{j,\gamma} {}^2D^{a,i,b,j} T_{c,i,d,j} V_{a,c,b,d} \quad (3331)$$

Factorized expression

$$\tau^0_{\gamma,\alpha,w} = \sum_{a \in V} {}^2D^1_{a,w} W^1_{a,\alpha} Y^{1,*}_{a,\gamma} \quad (3r_D r_T r_V N_v) \quad (3332)$$

$$\tau^1_{\gamma,\delta,w} = \sum_{a \in V} {}^2D^3_{a,w} Y^1_{a,\gamma} Y^{3,*}_{a,\delta} \quad (3r_D r_T^2 N_v) \quad (3333)$$

$$\tau^2_{\gamma,\alpha} = \sum_{i \in O} W^3_{i,\alpha} Y^2_{i,\gamma} \quad (2r_T r_V N_o) \quad (3334)$$

$$\tau^3_{\gamma,\alpha} = \sum_{a \in V} W^4_{a,\alpha} Y^3_{a,\gamma} \quad (2r_T r_V N_v) \quad (3335)$$

$$\tau^4_{\gamma,\alpha,i} = \sum_{\delta \in A} Z_{\gamma,\delta} Y^4_{i,\delta} \tau^3_{\delta,\alpha} \quad (3r_T^2 r_V N_o) \quad (3336)$$

$$\tau^5_{\gamma,\alpha,w} = \sum_{\delta \in A} \sum_{i \in O} {}^2D^4_{i,w} Y^{4,*}_{i,\gamma} \tau^2_{\delta,\alpha} \tau^1_{\delta,\gamma,w} \tau^4_{\delta,\alpha,i} \quad (5r_D r_T^2 r_V N_o) \quad (3337)$$

$$\tau^6_{\gamma,\alpha,w} = \sum_{\beta \in B} X_{\alpha,\beta} \tau^5_{\gamma,\beta,w} \quad (2r_D r_T r_V^2) \quad (3338)$$

$$\tau^7_{\gamma,\alpha,w} = \sum_{\delta \in A} Z^*_{\gamma,\delta} \tau^6_{\delta,\alpha,w} \quad (2r_D r_T^2 r_V) \quad (3339)$$

$$\tau^8_{\gamma,w,i} = \sum_{\alpha \in B} W^2_{i,\alpha} \tau^0_{\gamma,\alpha,w} \tau^7_{\gamma,\alpha,w} \quad (3r_D r_T r_V N_o) \quad (3340)$$

$${}^2R^2_{i,\gamma} \leftarrow - \sum_{w \in D} \frac{1}{2} {}^2D^2_{i,w} \tau^8_{\gamma,w,i} \quad (2r_D r_T N_o) \quad (3341)$$

Raw expression

$${}^2R^2_{i,\epsilon} \leftarrow \sum_{\gamma \in A} \sum_{j \in O} \sum_{a \in V} \sum_{b \in V} \sum_{c \in V} \sum_{d \in V} \frac{1}{2} Y^{1,*}_{a,\epsilon} Z^*_{\epsilon,\gamma} Y^{3,*}_{b,\gamma} Y^{4,*}_{j,\gamma} {}^2D^{a,i,b,j} T_{c,j,d,i} V_{a,d,b,c} \quad (3342)$$

Factorized expression

$$\tau^0_{\gamma,\alpha,w} = \sum_{a \in V} {}^2D^1_{a,w} W^1_{a,\alpha} Y^{1,*}_{a,\gamma} \quad (3r_D r_T r_V N_v) \quad (3343)$$

$$\tau^1_{\gamma,\delta,w} = \sum_{a \in V} {}^2D^3_{a,w} Y^3_{a,\gamma} Y^{3,*}_{a,\delta} \quad (3r_D r_T^2 N_v) \quad (3344)$$

$$\tau^2_{\gamma,\alpha} = \sum_{a \in V} W^4_{a,\alpha} Y^1_{a,\gamma} \quad (2r_T r_V N_v) \quad (3345)$$

$$\tau^3_{\gamma,\alpha,i} = \sum_{\delta \in A} Y^2_{i,\delta} Z_{\delta,\gamma} \tau^2_{\delta,\alpha} \quad (3r_T^2 r_V N_o) \quad (3346)$$

$$\tau^4_{\gamma,\alpha} = \sum_{i \in O} W^3_{i,\alpha} Y^4_{i,\gamma} \quad (2r_T r_V N_o) \quad (3347)$$

$$\tau^6_{\gamma,\alpha,i} = \sum_{j \in O} Y^2_{j,\gamma} \tau^5_{\alpha,j,i} \quad (2r_T r_V N_o^2) \quad (3360)$$

$$\tau^5_{\gamma,\alpha,w} = \sum_{\delta \in A} \sum_{i \in O} {}^2D^4_{i,w} Y^{4,*}_{i,\gamma} \tau^4_{\delta,\alpha} \tau^1_{\delta,\gamma,w} \tau^3_{\delta,\alpha,i} \quad (5r_D r_T^2 r_V N_o) \quad (3348)$$

$$\tau^6_{\gamma,\delta,w,i} = \sum_{\alpha \in B} \tau^6_{\gamma,\alpha,i} \tau^4_{\gamma,\delta,\alpha,w} \quad (2r_D r_T^2 r_V N_o) \quad (3361)$$

$$\tau^6_{\gamma,\alpha,w} = \sum_{\beta \in B} X_{\alpha,\beta} \tau^5_{\gamma,\beta,w} \quad (2r_D r_T r_V^2) \quad (3349)$$

$$\tau^8_{\gamma,\delta,i} = \sum_{\epsilon \in A} \sum_{w \in D} {}^2D^2_{i,w} \tau^0_{\epsilon,\gamma,w} \tau^7_{\epsilon,\delta,w,i} \quad (3r_D r_T^3 N_o) \quad (3362)$$

$$\tau^7_{\gamma,\alpha,w} = \sum_{\delta \in A} Z^*_{\gamma,\delta} \tau^6_{\delta,\alpha,w} \quad (2r_D r_T^2 r_V) \quad (3350)$$

$${}^2R^2_{i,\gamma} \leftarrow - \sum_{\delta \in A} \frac{1}{2} Z^*_{\gamma,\delta} \tau^8_{\gamma,\delta,i} \quad (2r_T^2 N_o) \quad (3363)$$

$$\tau^8_{\gamma,w,i} = \sum_{\alpha \in B} W^2_{i,\alpha} \tau^0_{\gamma,\alpha,w} \tau^7_{\gamma,\alpha,w} \quad (3r_D r_T r_V N_o) \quad (3351)$$

Raw expression

$${}^2R^2_{i,\epsilon} \leftarrow \sum_{\gamma \in A} \sum_{j \in O} \sum_{k \in O} \sum_{l \in O} \sum_{a \in V} \sum_{b \in V} \frac{1}{2} Y^{1,*}_{a,\epsilon} Z^*_{\epsilon,\gamma} Y^{3,*}_{b,\gamma} Y^{4,*}_{j,\gamma} {}^2D^{a,i,b,j} {}^2T_{b,k,a,l} V_{l,i,k,j} \quad (3364)$$

$${}^2R^2_{i,\gamma} \leftarrow - \sum_{w \in D} \frac{1}{2} {}^2D^2_{i,w} \tau^8_{\gamma,w,i} \quad (2r_D r_T N_o) \quad (3352)$$

Factorized expression

Raw expression

$${}^2R^2_{i,\epsilon} \leftarrow \sum_{\gamma \in A} \sum_{j \in O} \sum_{k \in O} \sum_{l \in O} \sum_{a \in V} \sum_{b \in V} \frac{1}{2} Y^{1,*}_{a,\epsilon} Z^*_{\epsilon,\gamma} Y^{3,*}_{b,\gamma} Y^{4,*}_{j,\gamma} {}^2D^{a,i,b,j} {}^2T_{a,k,b,l} V_{k,i,l,j} \quad (3353)$$

Factorized expression

$$\tau^0_{\gamma,\delta,w} = \sum_{a \in V} {}^2D^1_{a,w} Y^3_{a,\gamma} Y^{1,*}_{a,\delta} \quad (3r_D r_T^2 N_v) \quad (3365)$$

$$\tau^1_{\gamma,\alpha,w} = \sum_{a \in V} {}^2D^3_{a,w} W^1_{a,\alpha} Y^{3,*}_{a,\gamma} \quad (3r_D r_T r_V N_v) \quad (3366)$$

$$\tau^0_{\gamma,\delta,w} = \sum_{a \in V} {}^2D^1_{a,w} Y^1_{a,\gamma} Y^{1,*}_{a,\delta} \quad (3r_D r_T^2 N_v) \quad (3354)$$

$$\tau^2_{\gamma,\alpha} = \sum_{a \in V} W^2_{a,\alpha} Y^1_{a,\gamma} \quad (2r_T r_V N_v) \quad (3367)$$

$$\tau^1_{\gamma,\alpha,w} = \sum_{a \in V} {}^2D^3_{a,w} W^1_{a,\alpha} Y^{3,*}_{a,\gamma} \quad (3r_D r_T r_V N_v) \quad (3355)$$

$$\tau^3_{\gamma,\alpha,i} = \sum_{\delta \in A} Y^2_{i,\delta} Z_{\delta,\gamma} \tau^2_{\delta,\alpha} \quad (3r_T^2 r_V N_o) \quad (3368)$$

$$\tau^2_{\gamma,\alpha} = \sum_{a \in V} W^2_{a,\alpha} Y^3_{a,\gamma} \quad (2r_T r_V N_v) \quad (3356)$$

$$\tau^4_{\gamma,\delta,\alpha,w} = \sum_{i \in O} {}^2D^4_{i,w} Y^{4,*}_{i,\delta} \tau^1_{\delta,\alpha,w} \tau^3_{\gamma,\alpha,i} \quad (4r_D r_T^2 r_V N_o) \quad (3369)$$

$$\tau^3_{\gamma,\alpha,i} = \sum_{\delta \in A} Z_{\gamma,\delta} Y^4_{i,\delta} \tau^2_{\delta,\alpha} \quad (3r_T^2 r_V N_o) \quad (3357)$$

$$\tau^5_{\alpha,i,j} = \sum_{\beta \in B} X_{\alpha,\beta} W^3_{i,\beta} W^4_{j,\beta} \quad (3r_V^2 N_o^2) \quad (3370)$$

$$\tau^4_{\gamma,\delta,\alpha,w} = \sum_{i \in O} {}^2D^4_{i,w} Y^{4,*}_{i,\delta} \tau^1_{\delta,\alpha,w} \tau^3_{\gamma,\alpha,i} \quad (4r_D r_T^2 r_V N_o) \quad (3358)$$

$$\tau^6_{\gamma,\alpha,i} = \sum_{j \in O} Y^4_{j,\gamma} \tau^5_{\alpha,j,i} \quad (2r_T r_V N_o^2) \quad (3371)$$

$$\tau^5_{\alpha,i,j} = \sum_{\beta \in B} X_{\alpha,\beta} W^3_{i,\beta} W^4_{j,\beta} \quad (3r_V^2 N_o^2) \quad (3359)$$

$$\tau^7_{\gamma,\delta,w,i} = \sum_{\alpha \in B} \tau^6_{\gamma,\alpha,i} \tau^4_{\gamma,\delta,\alpha,w} \quad (2r_D r_T^2 r_V N_o) \quad (3372)$$

$$\tau^8_{\gamma,\delta,i} = \sum_{\epsilon \in A} \sum_{w \in D} {}^2D^2_{i,w} \tau^0_{\epsilon,\gamma,w} \tau^7_{\epsilon,\delta,w,i} \quad (3r_D r_T^3 N_o) \quad (3373)$$

$${}^2R^2_{i,\gamma} \leftarrow - \sum_{\delta \in A} \frac{1}{2} Z^*_{\gamma,\delta} \tau^8_{\gamma,\delta,i} \quad (2r_T^2 N_o) \quad (3374)$$

Raw expression

$${}^2R^2_{i,\epsilon} \leftarrow - \sum_{\gamma \in A} \sum_{j \in O} \sum_{k \in O} \sum_{a \in V} \sum_{b \in V} \frac{1}{2} Y^{1,*}_{a,\epsilon} Z^*_{\epsilon,\gamma} Y^{3,*}_{b,\gamma} Y^{4,*}_{j,\gamma} f_{k,i} {}^2D^{a,i,b,j} {}^2T_{a,k,b,j} \quad (3375)$$

Factorized expression

$$\tau^0_{\gamma,\delta,w} = \sum_{a \in V} {}^2D^1_{a,w} Y^1_{a,\gamma} Y^{1,*}_{a,\delta} \quad (3r_D r_T^2 N_v) \quad (3376)$$

$$\tau^1_{\alpha,i,j} = \sum_{\beta \in B} X_{\alpha,\beta} W^3_{i,\beta} W^4_{j,\beta} \quad (3r_V^2 N_o^2) \quad (3377)$$

$$\tau^2_{\gamma,\alpha,i} = \sum_{j \in O} Y^4_{j,\gamma} \tau^1_{\alpha,j,i} \quad (2r_T r_V N_o^2) \quad (3378)$$

$$\tau^3_{\gamma,\alpha} = \sum_{a \in V} W^2_{a,\alpha} Y^3_{a,\gamma} \quad (2r_T r_V N_v) \quad (3379)$$

$$\tau^4_{\gamma,i,a} = \sum_{\alpha \in B} W^1_{a,\alpha} \tau^3_{\gamma,\alpha} \tau^2_{\gamma,\alpha,i} \quad (3r_T r_V N_o N_v) \quad (3380)$$

$$\tau^5_{\gamma,\delta,w} = \sum_{i \in O} \sum_{a \in V} {}^2D^3_{a,w} {}^2D^4_{i,w} Y^{3,*}_{a,\delta} Y^{4,*}_{i,\delta} \tau^4_{\gamma,i,a} \quad (5r_D r_T^2 N_o N_v) \quad (3381)$$

$$\tau^6_{\gamma,\delta,w} = \sum_{\epsilon \in A} Z^*_{\delta,\epsilon} \tau^5_{\gamma,\epsilon,w} \quad (2r_D r_T^3) \quad (3382)$$

$$\tau^7_{\gamma,\delta,w} = \sum_{\epsilon \in A} Z_{\gamma,\epsilon} \tau^6_{\epsilon,\delta,w} \quad (2r_D r_T^3) \quad (3383)$$

$${}^2R^2_{i,\gamma} \leftarrow - \sum_{\delta \in A} \sum_{w \in D} \frac{1}{2} {}^2D^2_{i,w} Y^2_{i,\delta} \tau^0_{\delta,\gamma,w} \tau^7_{\delta,\gamma,w} \quad (4r_D r_T^2 N_o) \quad (3384)$$

Raw expression

$${}^2R^2_{i,\epsilon} \leftarrow - \sum_{\gamma \in A} \sum_{j \in O} \sum_{k \in O} \sum_{a \in V} \sum_{b \in V} \frac{1}{2} Y^{1,*}_{a,\epsilon} Z^*_{\epsilon,\gamma} Y^{3,*}_{b,\gamma} Y^{4,*}_{j,\gamma} f_{k,i} {}^2D^{a,i,b,j} {}^2T_{b,j,a,k} \quad (3385)$$

Factorized expression

$$\tau^0_{\gamma,\delta,w} = \sum_{a \in V} {}^2D^1_{a,w} Y^3_{a,\gamma} Y^{1,*}_{a,\delta} \quad (3r_D r_T^2 N_v) \quad (3386)$$

$$\tau^1_{\alpha,i,j} = \sum_{\beta \in B} X_{\alpha,\beta} W^3_{i,\beta} W^4_{j,\beta} \quad (3r_V^2 N_o^2) \quad (3387)$$

$$\tau^2_{\gamma,\alpha,i} = \sum_{j \in O} Y^2_{j,\gamma} \tau^1_{\alpha,j,i} \quad (2r_T r_V N_o^2) \quad (3388)$$

$$\tau^3_{\gamma,\alpha} = \sum_{a \in V} W^2_{a,\alpha} Y^1_{a,\gamma} \quad (2r_T r_V N_v) \quad (3389)$$

$$\tau^4_{\gamma,i,a} = \sum_{\alpha \in B} W^1_{a,\alpha} \tau^3_{\gamma,\alpha} \tau^2_{\gamma,\alpha,i} \quad (3r_T r_V N_o N_v) \quad (3390)$$

$$\tau^5_{\gamma,\delta,w} = \sum_{i \in O} \sum_{a \in V} {}^2D^3_{a,w} {}^2D^4_{i,w} Y^{3,*}_{a,\delta} Y^{4,*}_{i,\delta} \tau^4_{\gamma,i,a} \quad (5r_D r_T^2 N_o N_v) \quad (3391)$$

$$\tau^6_{\gamma,\delta,w} = \sum_{\epsilon \in A} Z^*_{\delta,\epsilon} \tau^5_{\gamma,\epsilon,w} \quad (2r_D r_T^3) \quad (3392)$$

$$\tau^7_{\gamma,\delta,w} = \sum_{\epsilon \in A} Z_{\epsilon,\gamma} \tau^6_{\epsilon,\delta,w} \quad (2r_D r_T^3) \quad (3393)$$

$${}^2R^2_{i,\gamma} \leftarrow - \sum_{\delta \in A} \sum_{w \in D} \frac{1}{2} {}^2D^2_{i,w} Y^4_{i,\delta} \tau^0_{\delta,\gamma,w} \tau^7_{\delta,\gamma,w} \quad (4r_D r_T^2 N_o) \quad (3394)$$

Raw expression

$${}^2R^2_{i,\epsilon} \leftarrow - \sum_{\gamma \in A} \sum_{j \in O} \sum_{k \in O} \sum_{a \in V} \sum_{b \in V} \frac{1}{2} Y^{1,*}_{a,\epsilon} Z^*_{\epsilon,\gamma} Y^{3,*}_{b,\gamma} Y^{4,*}_{j,\gamma} f_{k,j} {}^2D^{a,i,b,j} {}^2T_{a,i,b,k} \quad (3395)$$

Factorized expression

$$\tau^0_{\gamma,\delta,w} = \sum_{a \in V} {}^2D^1_{a,w} Y^1_{a,\gamma} Y^{1,*}_{a,\delta} \quad (3r_D r_T^2 N_v) \quad (3396)$$

$$\tau^1_{\gamma,\alpha} = \sum_{i \in O} W^3_{i,\alpha} Y^2_{i,\gamma} \quad (2r_T r_V N_o) \quad (3397)$$

$$\tau^2_{\gamma,\alpha} = \sum_{a \in V} W^4_{a,\alpha} Y^3_{a,\gamma} \quad (2r_T r_V N_v) \quad (3398)$$

$$\tau^3_{\gamma,\alpha,i} = \sum_{\delta \in A} Z_{\gamma,\delta} Y^4_{i,\delta} \tau^2_{\delta,\alpha} \quad (3r_T^2 r_V N_o) \quad (3399)$$

$$\tau^4_{\gamma,\alpha,w} = \sum_{a \in V} {}^2D^3_{a,w} W^1_{a,\alpha} Y^{3,*}_{a,\gamma} \quad (3r_D r_T r_V N_v) \quad (3400)$$

$$\tau^5_{\gamma,\alpha,w} = \sum_{i \in O} {}^2D^4_{i,w} W^2_{i,\alpha} Y^{4,*}_{i,\gamma} \quad (3r_D r_T r_V N_o) \quad (3401)$$

$$\tau^6_{\gamma,\alpha,w} = \sum_{\beta \in B} X_{\beta,\alpha} \tau^4_{\gamma,\beta,w} \tau^5_{\gamma,\beta,w} \quad (3r_D r_T r_V^2) \quad (3402)$$

$$\tau^7_{\gamma,\alpha,w} = \sum_{\delta \in A} Z^*_{\gamma,\delta} \tau^6_{\delta,\alpha,w} \quad (2r_D r_T^2 r_V) \quad (3403)$$

$$\tau^8_{\gamma,\delta,w,i} = \sum_{\alpha \in B} \tau^1_{\gamma,\alpha} \tau^3_{\gamma,\alpha,i} \tau^7_{\delta,\alpha,w} \quad (3r_D r_T^2 r_V N_o) \quad (3404)$$

$$\tau^9_{\gamma,w,i} = \sum_{\delta \in A} \tau^0_{\delta,\gamma,w} \tau^8_{\delta,\gamma,w,i} \quad (2r_D r_T^2 N_o) \quad (3405)$$

$${}^2R^2_{i,\gamma} \leftarrow - \sum_{w \in D} \frac{1}{2} {}^2D^2_{i,w} \tau^9_{\gamma,w,i} \quad (2r_D r_T N_o) \quad (3406)$$

Raw expression

$${}^2R^2_{i,\epsilon} \leftarrow - \sum_{\gamma \in A} \sum_{j \in O} \sum_{k \in O} \sum_{a \in V} \sum_{b \in V} \frac{1}{2} Y^{1,*}_{a,\epsilon} Z^*_{\epsilon,\gamma} Y^{3,*}_{b,\gamma} Y^{4,*}_{j,\gamma} f_{k,j} {}^2D^{a,i,b,j} {}^2T_{b,k,a,i} \quad (3407)$$

Factorized expression

$$\tau^0_{\gamma,\delta,w} = \sum_{a \in V} {}^2D^1_{a,w} Y^3_{a,\gamma} Y^{1,*}_{a,\delta} \quad (3r_D r_T^2 N_v) \quad (3408)$$

$$\tau^1_{\gamma,\alpha} = \sum_{a \in V} W^4_{a,\alpha} Y^1_{a,\gamma} \quad (2r_T r_V N_v) \quad (3409)$$

$$\tau^2_{\gamma,\alpha,i} = \sum_{\delta \in A} Y^2_{i,\delta} Z_{\delta,\gamma} \tau^1_{\delta,\alpha} \quad (3r_T^2 r_V N_o) \quad (3410)$$

$$\tau^3_{\gamma,\alpha} = \sum_{i \in O} W^3_{i,\alpha} Y^4_{i,\gamma} \quad (2r_T r_V N_o) \quad (3411)$$

$$\tau^4_{\gamma,\alpha,w} = \sum_{a \in V} {}^2D^3_{a,w} W^1_{a,\alpha} Y^{3,*}_{a,\gamma} \quad (3r_D r_T r_V N_v) \quad (3412)$$

$$\tau^5_{\gamma,\alpha,w} = \sum_{i \in O} {}^2D^4_{i,w} W^2_{i,\alpha} Y^{4,*}_{i,\gamma} \quad (3r_D r_T r_V N_o) \quad (3413)$$

$$\tau^6_{\gamma,\alpha,w} = \sum_{\beta \in B} X_{\beta,\alpha} \tau^4_{\gamma,\beta,w} \tau^5_{\gamma,\beta,w} \quad (3r_D r_T r_V^2) \quad (3414)$$

$$\tau^7_{\gamma,\alpha,w} = \sum_{\delta \in A} Z^*_{\gamma,\delta} \tau^6_{\delta,\alpha,w} \quad (2r_D r_T^2 r_V) \quad (3415)$$

$$\tau^8_{\gamma,\delta,w,i} = \sum_{\alpha \in B} \tau^3_{\gamma,\alpha} \tau^2_{\gamma,\alpha,i} \tau^7_{\delta,\alpha,w} \quad (3r_D r_T^2 r_V N_o) \quad (3416)$$

$$\tau^9_{\gamma,w,i} = \sum_{\delta \in A} \tau^0_{\delta,\gamma,w} \tau^8_{\delta,\gamma,w,i} \quad (2r_D r_T^2 N_o) \quad (3417)$$

$${}^2R^2_{i,\gamma} \leftarrow - \sum_{w \in D} \frac{1}{2} {}^2D^2_{i,w} \tau^9_{\gamma,w,i} \quad (2r_D r_T N_o) \quad (3418)$$

## E. Contributions from $(H^1 T^1 T^1 T)_c$

Raw expression

$${}^2R^2_{i,\epsilon} \leftarrow - \sum_{\gamma \in A} \sum_{j \in O} \sum_{k \in O} \sum_{a \in V} \sum_{b \in V} \sum_{c \in V} \sum_{d \in V} {}^1T_{a,k} {}^1T_{c,i} {}^1T_{d,j} Y^{1,*}_{a,\epsilon} Z^*_{\epsilon,\gamma} Y^{3,*}_{b,\gamma} Y^{4,*}_{j,\gamma} {}^2D^{a,i,b,j} V_{b,d,k,c} \quad (3419)$$

Factorized expression

$$\tau^0_{\alpha,i} = \sum_{a \in V} {}^1T_{a,i} W^2_{a,\alpha} \quad (2r_V N_o N_v) \quad (3420)$$

$$\tau^1_{\gamma,\alpha,w} = \sum_{i \in O} {}^2D^4_{i,w} Y^{4,*}_{i,\gamma} \tau^0_{\alpha,i} \quad (3r_D r_T r_V N_o) \quad (3421)$$

$$\tau_{\gamma,\alpha,w}^2 = \sum_{a \in V} {}^2D_{a,w}^3 W_{a,\alpha}^1 Y_{a,\gamma}^{3,*} \quad (3r_D r_T r_V N_v) \quad (3422)$$

$$\tau_{\gamma,w,i}^3 = \sum_{a \in V} {}^2D_{a,w}^3 {}^1T_{a,i} Y_{a,\gamma}^{3,*} \quad (3r_D r_T N_o N_v) \quad (3434)$$

$$\tau_{\gamma,\alpha,w}^3 = \sum_{\beta \in B} X_{\beta,\alpha} \tau_{\gamma,\beta,w}^1 \tau_{\gamma,\beta,w}^2 \quad (3r_D r_T r_V^2) \quad (3423)$$

$$\tau_{\gamma,\alpha,w}^4 = \sum_{i \in O} W_{i,\alpha}^3 \tau_{\gamma,w,i}^3 \quad (2r_D r_T r_V N_o) \quad (3435)$$

$$\tau_{\gamma,\alpha,w}^4 = \sum_{\delta \in A} Z_{\gamma,\delta}^* \tau_{\delta,\alpha,w}^3 \quad (2r_D r_T^2 r_V) \quad (3424)$$

$$\tau_{\gamma,\alpha,w}^5 = \sum_{\beta \in B} X_{\alpha,\beta} \tau_{\gamma,\beta,w}^2 \tau_{\gamma,\beta,w}^4 \quad (3r_D r_T r_V^2) \quad (3436)$$

$$\tau_{\gamma,w,i}^5 = \sum_{a \in V} {}^2D_{a,w}^1 {}^1T_{a,i} Y_{a,\gamma}^{1,*} \quad (3r_D r_T N_o N_v) \quad (3425)$$

$$\tau_{\gamma,\alpha,w}^6 = \sum_{\delta \in A} Z_{\gamma,\delta}^* \tau_{\delta,\alpha,w}^5 \quad (2r_D r_T^2 r_V) \quad (3437)$$

$$\tau_{\gamma,\alpha,w}^6 = \sum_{i \in O} W_{i,\alpha}^3 \tau_{\gamma,w,i}^5 \quad (2r_D r_T r_V N_o) \quad (3426)$$

$$\tau_{\alpha,i}^7 = \sum_{a \in V} {}^1T_{a,i} W_{a,\alpha}^2 \quad (2r_V N_o N_v) \quad (3438)$$

$$\tau_{\alpha,i}^7 = \sum_{a \in V} {}^1T_{a,i} W_{a,\alpha}^4 \quad (2r_V N_o N_v) \quad (3427)$$

$$\tau_{\gamma,w,i}^8 = \sum_{\alpha \in B} \tau_{\alpha,i}^7 \tau_{\gamma,\alpha,w}^0 \tau_{\gamma,\alpha,w}^6 \quad (3r_D r_T r_V N_o) \quad (3439)$$

$$\tau_{\gamma,w,i}^8 = \sum_{\alpha \in B} \tau_{\alpha,i}^7 \tau_{\gamma,\alpha,w}^4 \tau_{\gamma,\alpha,w}^6 \quad (3r_D r_T r_V N_o) \quad (3428)$$

$${}^2R_{i,\gamma}^2 \leftarrow - \sum_{w \in D} {}^2D_{i,w}^2 \tau_{\gamma,w,i}^8 \quad (2r_D r_T N_o) \quad (3440)$$

$${}^2R_{i,\gamma}^2 \leftarrow - \sum_{w \in D} {}^2D_{i,w}^2 \tau_{\gamma,w,i}^8 \quad (2r_D r_T N_o) \quad (3429)$$

Raw expression

$${}^2R_{i,\epsilon}^2 \leftarrow \sum_{\gamma \in A} \sum_{j \in O} \sum_{k \in O} \sum_{l \in O} \sum_{a \in V} \sum_{b \in V} \sum_{c \in V} {}^1T_{a,k} {}^1T_{b,l} {}^1T_{c,i} Y_{a,\epsilon}^{1,*} Z_{\epsilon,\gamma}^* Y_{b,\gamma}^{3,*} Y_{j,\gamma}^{4,*} {}^2D_{a,i,b,j} V_{k,c,l,j} \quad (3441)$$

Raw expression

$${}^2R_{i,\epsilon}^2 \leftarrow - \sum_{\gamma \in A} \sum_{j \in O} \sum_{k \in O} \sum_{a \in V} \sum_{b \in V} \sum_{c \in V} \sum_{d \in V} {}^1T_{b,k} {}^1T_{c,i} {}^1T_{d,j} Y_{a,\epsilon}^{1,*} Z_{\epsilon,\gamma}^* Y_{b,\gamma}^{3,*} Y_{j,\gamma}^{4,*} {}^2D_{a,i,b,j} V_{a,c,k,d} \quad (3430)$$

Factorized expression

$$\tau_{\gamma,w,i}^0 = \sum_{a \in V} {}^2D_{a,w}^3 {}^1T_{a,i} Y_{a,\gamma}^{3,*} \quad (3r_D r_T N_o N_v) \quad (3442)$$

Factorized expression

$$\tau_{\gamma,\alpha,w}^0 = \sum_{a \in V} {}^2D_{a,w}^1 W_{a,\alpha}^1 Y_{a,\gamma}^{1,*} \quad (3r_D r_T r_V N_v) \quad (3431)$$

$$\tau_{\gamma,\alpha,w}^1 = \sum_{i \in O} W_{i,\alpha}^3 \tau_{\gamma,w,i}^0 \quad (2r_D r_T r_V N_o) \quad (3443)$$

$$\tau_{\alpha,i}^1 = \sum_{a \in V} {}^1T_{a,i} W_{a,\alpha}^4 \quad (2r_V N_o N_v) \quad (3432)$$

$$\tau_{\gamma,\alpha,w}^2 = \sum_{i \in O} {}^2D_{i,w}^4 W_{i,\alpha}^4 Y_{i,\gamma}^{4,*} \quad (3r_D r_T r_V N_o) \quad (3444)$$

$$\tau_{\gamma,\alpha,w}^2 = \sum_{i \in O} {}^2D_{i,w}^4 Y_{i,\gamma}^{4,*} \tau_{\alpha,i}^1 \quad (3r_D r_T r_V N_o) \quad (3433)$$

$$\tau_{\gamma,\alpha,w}^3 = \sum_{\beta \in B} X_{\alpha,\beta} \tau_{\gamma,\beta,w}^1 \tau_{\gamma,\beta,w}^2 \quad (3r_D r_T r_V^2) \quad (3445)$$



$$\tau^4_{\gamma,\alpha,w} = \sum_{\delta \in A} Z^*_{\gamma,\delta} \tau^3_{\delta,\alpha,w} \quad (2r_D r_T^2 r_V) \quad (3446)$$

$$\tau^5_{\gamma,w,i} = \sum_{a \in V} {}^2D^1_{a,w} {}^1T_{a,i} Y^{1,*}_{a,\gamma} \quad (3r_D r_T N_o N_v) \quad (3447)$$

$$\tau^6_{\gamma,\alpha,w} = \sum_{i \in O} W^1_{i,\alpha} \tau^5_{\gamma,w,i} \quad (2r_D r_T r_V N_o) \quad (3448)$$

$$\tau^7_{\alpha,i} = \sum_{a \in V} {}^1T_{a,i} W^2_{a,\alpha} \quad (2r_V N_o N_v) \quad (3449)$$

$$\tau^8_{\gamma,w,i} = \sum_{\alpha \in B} \tau^7_{\alpha,i} \tau^4_{\gamma,\alpha,w} \tau^6_{\gamma,\alpha,w} \quad (3r_D r_T r_V N_o) \quad (3450)$$

$${}^2R^2_{i,\gamma} \leftarrow \sum_{w \in D} {}^2D^2_{i,w} \tau^8_{\gamma,w,i} \quad (2r_D r_T N_o) \quad (3451)$$

Raw expression

$${}^2R^2_{i,\epsilon} \leftarrow \sum_{\gamma \in A} \sum_{j \in O} \sum_{k \in O} \sum_{l \in O} \sum_{a \in V} \sum_{b \in V} \sum_{c \in V} {}^1T_{a,k} {}^1T_{b,l} {}^1T_{c,j} Y^{1,*}_{a,\epsilon} Z^*_{\epsilon,\gamma} Y^{3,*}_{b,\gamma} Y^{4,*}_{j,\gamma} {}^2D^{a,i,b,j} V_{k,i,l,c} \quad (3452)$$

Factorized expression

$$\tau^0_{\alpha,i} = \sum_{a \in V} {}^1T_{a,i} W^4_{a,\alpha} \quad (2r_V N_o N_v) \quad (3453)$$

$$\tau^1_{\gamma,\alpha,w} = \sum_{i \in O} {}^2D^4_{i,w} Y^{4,*}_{i,\gamma} \tau^0_{\alpha,i} \quad (3r_D r_T r_V N_o) \quad (3454)$$

$$\tau^2_{\gamma,w,i} = \sum_{a \in V} {}^2D^3_{a,w} {}^1T_{a,i} Y^{3,*}_{a,\gamma} \quad (3r_D r_T N_o N_v) \quad (3455)$$

$$\tau^3_{\gamma,\alpha,w} = \sum_{i \in O} W^3_{i,\alpha} \tau^2_{\gamma,w,i} \quad (2r_D r_T r_V N_o) \quad (3456)$$

$$\tau^4_{\gamma,\alpha,w} = \sum_{\beta \in B} X_{\alpha,\beta} \tau^1_{\gamma,\beta,w} \tau^3_{\gamma,\beta,w} \quad (3r_D r_T r_V^2) \quad (3457)$$

$$\tau^5_{\gamma,\alpha,w} = \sum_{\delta \in A} Z^*_{\gamma,\delta} \tau^4_{\delta,\alpha,w} \quad (2r_D r_T^2 r_V) \quad (3458)$$

$$\tau^6_{\gamma,w,i} = \sum_{a \in V} {}^2D^1_{a,w} {}^1T_{a,i} Y^{1,*}_{a,\gamma} \quad (3r_D r_T N_o N_v) \quad (3459)$$

$$\tau^7_{\gamma,\alpha,w} = \sum_{i \in O} W^1_{i,\alpha} \tau^6_{\gamma,w,i} \quad (2r_D r_T r_V N_o) \quad (3460)$$

$$\tau^8_{\gamma,w,i} = \sum_{\alpha \in B} W^2_{i,\alpha} \tau^5_{\gamma,\alpha,w} \tau^7_{\gamma,\alpha,w} \quad (3r_D r_T r_V N_o) \quad (3461)$$

$${}^2R^2_{i,\gamma} \leftarrow \sum_{w \in D} {}^2D^2_{i,w} \tau^8_{\gamma,w,i} \quad (2r_D r_T N_o) \quad (3462)$$

## F. Contributions from $(H^1 T^2 T)_c$

Raw expression

$${}^2R^2_{i,\epsilon} \leftarrow - \sum_{\gamma \in A} \sum_{j \in O} \sum_{k \in O} \sum_{a \in V} \sum_{b \in V} \sum_{c \in V} \frac{1}{2} {}^1T_{a,k} Y^{1,*}_{a,\epsilon} Z^*_{\epsilon,\gamma} Y^{3,*}_{b,\gamma} Y^{4,*}_{j,\gamma} f_{k,c} {}^2D^{a,i,b,j} {}^2T_{b,j,c,i} \quad (3463)$$

Factorized expression

$$\tau^0_{\gamma,w,i} = \sum_{a \in V} {}^2D^1_{a,w} {}^1T_{a,i} Y^{1,*}_{a,\gamma} \quad (3r_D r_T N_o N_v) \quad (3464)$$

$$\tau^1_{\gamma,i} = \sum_{a \in V} Y^3_{a,\gamma} f_{i,a} \quad (2r_T N_o N_v) \quad (3465)$$

$$\tau^2_{\gamma,\delta,w} = \sum_{i \in O} \tau^1_{\gamma,i} \tau^0_{\delta,w,i} \quad (2r_D r_T^2 N_o) \quad (3466)$$

$$\tau^3_{\gamma,\delta,w} = \sum_{a \in V} {}^2D^3_{a,w} Y^1_{a,\gamma} Y^{3,*}_{a,\delta} \quad (3r_D r_T^2 N_v) \quad (3467)$$

$$\tau^4_{\gamma,\delta,w} = \sum_{i \in O} {}^2D^4_{i,w} Y^2_{i,\gamma} Y^{4,*}_{i,\delta} \quad (3r_D r_T^2 N_o) \quad (3468)$$

$$\tau^5_{\gamma,\delta,w} = \sum_{\epsilon \in A} Z^*_{\delta,\epsilon} \tau^3_{\gamma,\epsilon,w} \tau^4_{\gamma,\epsilon,w} \quad (3r_D r_T^3) \quad (3469)$$

$$\tau^6_{\gamma,\delta,w} = \sum_{\epsilon \in A} Z_{\epsilon,\gamma} \tau^5_{\epsilon,\delta,w} \quad (2r_D r_T^3) \quad (3470)$$

$${}^2R^2_{i,\gamma} \leftarrow - \sum_{\delta \in A} \sum_{w \in D} \frac{1}{2} {}^2D^2_{i,w} Y^4_{i,\delta} \tau^2_{\delta,\gamma,w} \tau^6_{\delta,\gamma,w} \quad (4r_D r_T^2 N_o) \tau^0_{\gamma,\delta,w} = \sum_{a \in V} {}^2D^1_{a,w} Y^1_{a,\gamma} Y^{1,*}_{a,\delta} \quad (3r_D r_T^2 N_v) \quad (3482)$$

$$(3471)$$

Raw expression

$$\tau^1_{\gamma,\delta,w} = \sum_{i \in O} {}^2D^4_{i,w} Y^4_{i,\gamma} Y^{4,*}_{i,\delta} \quad (3r_D r_T^2 N_o) \quad (3483)$$

$${}^2R^2_{i,\epsilon} \leftarrow - \sum_{\gamma \in A} \sum_{j \in O} \sum_{k \in O} \sum_{a \in V} \sum_{b \in V} \sum_{c \in V} \frac{1}{2} {}^1T_{a,k} Y^{1,*}_{a,\epsilon} Z^*_{\epsilon,\gamma} Y^{3,*}_{b,\gamma} Y^{4,*}_{j,\gamma} f_{k,c} {}^2D^{a,i,b,j} {}^2T_{c,i,b,j} \quad (3472)$$

$$\tau^2_{\gamma,w,i} = \sum_{a \in V} {}^2D^3_{a,w} {}^1T_{a,i} Y^{3,*}_{a,\gamma} \quad (3r_D r_T N_o N_v) \quad (3484)$$

Factorized expression

$$\tau^3_{\gamma,i} = \sum_{a \in V} Y^3_{a,\gamma} f_{i,a} \quad (2r_T N_o N_v) \quad (3485)$$

$$\tau^0_{\gamma,w,i} = \sum_{a \in V} {}^2D^1_{a,w} {}^1T_{a,i} Y^{1,*}_{a,\gamma} \quad (3r_D r_T N_o N_v) \quad (3473)$$

$$\tau^4_{\gamma,\delta,w} = \sum_{i \in O} \tau^3_{\gamma,i} \tau^2_{\delta,w,i} \quad (2r_D r_T^2 N_o) \quad (3486)$$

$$\tau^1_{\gamma,i} = \sum_{a \in V} Y^1_{a,\gamma} f_{i,a} \quad (2r_T N_o N_v) \quad (3474)$$

$$\tau^5_{\gamma,\delta,w} = \sum_{\epsilon \in A} Z^*_{\delta,\epsilon} \tau^1_{\gamma,\epsilon,w} \tau^4_{\gamma,\epsilon,w} \quad (3r_D r_T^3) \quad (3487)$$

$$\tau^2_{\gamma,\delta,w} = \sum_{i \in O} \tau^1_{\gamma,i} \tau^0_{\delta,w,i} \quad (2r_D r_T^2 N_o) \quad (3475)$$

$$\tau^6_{\gamma,\delta,w} = \sum_{\epsilon \in A} Z_{\gamma,\epsilon} \tau^5_{\epsilon,\delta,w} \quad (2r_D r_T^3) \quad (3488)$$

$$\tau^3_{\gamma,\delta,w} = \sum_{a \in V} {}^2D^3_{a,w} Y^3_{a,\gamma} Y^{3,*}_{a,\delta} \quad (3r_D r_T^2 N_v) \quad (3476)$$

$${}^2R^2_{i,\gamma} \leftarrow - \sum_{\delta \in A} \sum_{w \in D} \frac{1}{2} {}^2D^2_{i,w} Y^2_{i,\delta} \tau^0_{\delta,\gamma,w} \tau^6_{\delta,\gamma,w} \quad (4r_D r_T^2 N_o) \quad (3489)$$

$$\tau^4_{\gamma,\delta,w} = \sum_{i \in O} {}^2D^4_{i,w} Y^4_{i,\gamma} Y^{4,*}_{i,\delta} \quad (3r_D r_T^2 N_o) \quad (3477)$$

Raw expression

$$\tau^5_{\gamma,\delta,w} = \sum_{\epsilon \in A} Z^*_{\delta,\epsilon} \tau^3_{\gamma,\epsilon,w} \tau^4_{\gamma,\epsilon,w} \quad (3r_D r_T^3) \quad (3478)$$

$${}^2R^2_{i,\epsilon} \leftarrow - \sum_{\gamma \in A} \sum_{j \in O} \sum_{k \in O} \sum_{a \in V} \sum_{b \in V} \sum_{c \in V} \frac{1}{2} {}^1T_{b,k} Y^{1,*}_{a,\epsilon} Z^*_{\epsilon,\gamma} Y^{3,*}_{b,\gamma} Y^{4,*}_{j,\gamma} f_{k,c} {}^2D^{a,i,b,j} {}^2T_{c,j,a,i} \quad (3490)$$

$$\tau^6_{\gamma,\delta,w} = \sum_{\epsilon \in A} Z_{\gamma,\epsilon} \tau^5_{\epsilon,\delta,w} \quad (2r_D r_T^3) \quad (3479)$$

Factorized expression

$$\tau^0_{\gamma,\delta,w} = \sum_{a \in V} {}^2D^1_{a,w} Y^3_{a,\gamma} Y^{1,*}_{a,\delta} \quad (3r_D r_T^2 N_v) \quad (3491)$$

$${}^2R^2_{i,\gamma} \leftarrow - \sum_{\delta \in A} \sum_{w \in D} \frac{1}{2} {}^2D^2_{i,w} Y^2_{i,\delta} \tau^2_{\delta,\gamma,w} \tau^6_{\delta,\gamma,w} \quad (4r_D r_T^2 N_o) \quad (3480)$$

$$\tau^1_{\gamma,\delta,w} = \sum_{i \in O} {}^2D^4_{i,w} Y^2_{i,\gamma} Y^{4,*}_{i,\delta} \quad (3r_D r_T^2 N_o) \quad (3492)$$

Raw expression

$${}^2R^2_{i,\epsilon} \leftarrow - \sum_{\gamma \in A} \sum_{j \in O} \sum_{k \in O} \sum_{a \in V} \sum_{b \in V} \sum_{c \in V} \frac{1}{2} {}^1T_{b,k} Y^{1,*}_{a,\epsilon} Z^*_{\epsilon,\gamma} Y^{3,*}_{b,\gamma} Y^{4,*}_{j,\gamma} f_{k,c} {}^2D^{a,i,b,j} {}^2T_{a,i,c,j} \quad (3481)$$

$$\tau^2_{\gamma,w,i} = \sum_{a \in V} {}^2D^3_{a,w} {}^1T_{a,i} Y^{3,*}_{a,\gamma} \quad (3r_D r_T N_o N_v) \quad (3493)$$

Factorized expression

$$\tau^3_{\gamma,i} = \sum_{a \in V} Y^1_{a,\gamma} f_{i,a} \quad (2r_T N_o N_v) \quad (3494)$$

$$\tau^4_{\gamma,\delta,w} = \sum_{i \in O} \tau^3_{\gamma,i} \tau^2_{\delta,w,i} \quad (2r_D r_T^2 N_o) \quad (3495)$$

$$\tau^5_{\gamma,\delta,w} = \sum_{\epsilon \in A} Z^*_{\delta,\epsilon} \tau^1_{\gamma,\epsilon,w} \tau^4_{\gamma,\epsilon,w} \quad (3r_D r_T^3) \quad (3496)$$

$$\tau^6_{\gamma,\delta,w} = \sum_{\epsilon \in A} Z_{\epsilon,\gamma} \tau^5_{\epsilon,\delta,w} \quad (2r_D r_T^3) \quad (3497)$$

$${}^2R^2_{i,\gamma} \leftarrow - \sum_{\delta \in A} \sum_{w \in D} \frac{1}{2} {}^2D^2_{i,w} Y^4_{i,\delta} \tau^0_{\delta,\gamma,w} \tau^6_{\delta,\gamma,w} \quad (4r_D r_T^2 N_o) \quad (3498)$$

Raw expression

$${}^2R^2_{i,\epsilon} \leftarrow - \sum_{\gamma \in A} \sum_{j \in O} \sum_{k \in O} \sum_{a \in V} \sum_{b \in V} \sum_{c \in V} \frac{1}{2} {}^1T_{c,i} Y^{1,*}_{a,\epsilon} Z^*_{\epsilon,\gamma} Y^{3,*}_{b,\gamma} Y^{4,*}_{j,\gamma} f_{k,c} {}^2D^{a,i,b,j} {}^2T_{a,k,b,j} \quad (3499)$$

Factorized expression

$$\tau^0_{\gamma,\delta,w} = \sum_{a \in V} {}^2D^1_{a,w} Y^1_{a,\gamma} Y^{1,*}_{a,\delta} \quad (3r_D r_T^2 N_v) \quad (3500)$$

$$\tau^1_{\gamma,\delta,w} = \sum_{a \in V} {}^2D^3_{a,w} Y^3_{a,\gamma} Y^{3,*}_{a,\delta} \quad (3r_D r_T^2 N_v) \quad (3501)$$

$$\tau^2_{\gamma,\delta,w} = \sum_{i \in O} {}^2D^4_{i,w} Y^4_{i,\gamma} Y^{4,*}_{i,\delta} \quad (3r_D r_T^2 N_o) \quad (3502)$$

$$\tau^3_{\gamma,\delta,w} = \sum_{\epsilon \in A} Z^*_{\delta,\epsilon} \tau^1_{\gamma,\epsilon,w} \tau^2_{\gamma,\epsilon,w} \quad (3r_D r_T^3) \quad (3503)$$

$$\tau^4_{\gamma,\delta,w} = \sum_{\epsilon \in A} Z_{\gamma,\epsilon} \tau^3_{\epsilon,\delta,w} \quad (2r_D r_T^3) \quad (3504)$$

$$\tau^5_{i,j} = \sum_{a \in V} {}^1T_{a,i} f_{j,a} \quad (2N_o {}^2N_v) \quad (3505)$$

$$\tau^6_{\gamma,i} = \sum_{j \in O} Y^2_{j,\gamma} \tau^5_{i,j} \quad (2r_T N_o^2) \quad (3506)$$

$${}^2R^2_{i,\gamma} \leftarrow - \sum_{\delta \in A} \sum_{w \in D} \frac{1}{2} {}^2D^2_{i,w} \tau^6_{\delta,i} \tau^0_{\delta,\gamma,w} \tau^4_{\delta,\gamma,w} \quad (4r_D r_T^2 N_o) \quad (3507)$$

Raw expression

$${}^2R^2_{i,\epsilon} \leftarrow - \sum_{\gamma \in A} \sum_{j \in O} \sum_{k \in O} \sum_{a \in V} \sum_{b \in V} \sum_{c \in V} \frac{1}{2} {}^1T_{c,i} Y^{1,*}_{a,\epsilon} Z^*_{\epsilon,\gamma} Y^{3,*}_{b,\gamma} Y^{4,*}_{j,\gamma} f_{k,c} {}^2D^{a,i,b,j} {}^2T_{b,j,a,k} \quad (3508)$$

Factorized expression

$$\tau^0_{\gamma,\delta,w} = \sum_{a \in V} {}^2D^3_{a,w} Y^1_{a,\gamma} Y^{3,*}_{a,\delta} \quad (3r_D r_T^2 N_v) \quad (3509)$$

$$\tau^1_{\gamma,\delta,w} = \sum_{i \in O} {}^2D^4_{i,w} Y^2_{i,\gamma} Y^{4,*}_{i,\delta} \quad (3r_D r_T^2 N_o) \quad (3510)$$

$$\tau^2_{\gamma,\delta,w} = \sum_{\epsilon \in A} Z^*_{\delta,\epsilon} \tau^0_{\gamma,\epsilon,w} \tau^1_{\gamma,\epsilon,w} \quad (3r_D r_T^3) \quad (3511)$$

$$\tau^3_{\gamma,\delta,w} = \sum_{\epsilon \in A} Z_{\epsilon,\gamma} \tau^2_{\epsilon,\delta,w} \quad (2r_D r_T^3) \quad (3512)$$

$$\tau^4_{\gamma,\delta,w} = \sum_{a \in V} {}^2D^1_{a,w} Y^3_{a,\gamma} Y^{1,*}_{a,\delta} \quad (3r_D r_T^2 N_v) \quad (3513)$$

$$\tau^5_{i,j} = \sum_{a \in V} {}^1T_{a,i} f_{j,a} \quad (2N_o {}^2N_v) \quad (3514)$$

$$\tau^6_{\gamma,i} = \sum_{j \in O} Y^4_{j,\gamma} \tau^5_{i,j} \quad (2r_T N_o^2) \quad (3515)$$

$${}^2R^2_{i,\gamma} \leftarrow - \sum_{\delta \in A} \sum_{w \in D} \frac{1}{2} {}^2D^2_{i,w} \tau^6_{\delta,i} \tau^3_{\delta,\gamma,w} \tau^4_{\delta,\gamma,w} \quad (4r_D r_T^2 N_o) \quad (3516)$$

Raw expression

$${}^2R^2_{i,\epsilon} \leftarrow - \sum_{\gamma \in A} \sum_{j \in O} \sum_{k \in O} \sum_{a \in V} \sum_{b \in V} \sum_{c \in V} \frac{1}{2} {}^1T_{c,j} Y^{1,*}_{a,\epsilon} Z^*_{\epsilon,\gamma} Y^{3,*}_{b,\gamma} Y^{4,*}_{j,\gamma} f_{k,c} {}^2D^{a,i,b,j} {}^2T_{a,i,b,k} \quad (3517)$$

Factorized expression

$$\tau^0_{\gamma,\delta,w} = \sum_{a \in V} {}^2D^1_{a,w} Y^1_{a,\gamma} Y^{1,*}_{a,\delta} \quad (3r_D r_T^2 N_v) \quad (3518)$$

$$\tau^1_{\gamma,\delta,w} = \sum_{a \in V} {}^2D^3_{a,w} Y^3_{a,\gamma} Y^{3,*}_{a,\delta} \quad (3r_D r_T^2 N_v) \quad (3519)$$

$$\tau^2_{i,j} = \sum_{a \in V} {}^1T_{a,i} f_{j,a} \quad (2N_o^2 N_v) \quad (3520)$$

$$\tau^6_{\gamma,\delta,w} = \sum_{\epsilon \in A} Z_{\epsilon,\gamma} \tau^5_{\epsilon,\delta,w} \quad (2r_D r_T^3) \quad (3533)$$

$$\tau^3_{\gamma,i} = \sum_{j \in O} Y^4_{j,\gamma} \tau^2_{i,j} \quad (2r_T N_o^2) \quad (3521)$$

$${}^2R^2_{i,\gamma} \leftarrow - \sum_{\delta \in A} \sum_{w \in D} \frac{1}{2} {}^2D^2_{i,w} Y^4_{i,\delta} \tau^0_{\delta,\gamma,w} \tau^6_{\delta,\gamma,w} \quad (4r_D r_T^2 N_o) \quad (3534)$$

$$\tau^4_{\gamma,\delta,w} = \sum_{i \in O} {}^2D^4_{i,w} Y^{4,*}_{i,\delta} \tau^3_{\gamma,i} \quad (3r_D r_T^2 N_o) \quad (3522)$$

Raw expression

$$\tau^5_{\gamma,\delta,w} = \sum_{\epsilon \in A} Z^*_{\delta,\epsilon} \tau^1_{\gamma,\epsilon,w} \tau^4_{\gamma,\epsilon,w} \quad (3r_D r_T^3) \quad (3523)$$

$${}^2R^2_{i,\epsilon} \leftarrow \sum_{\gamma \in A} \sum_{j \in O} \sum_{k \in O} \sum_{a \in V} \sum_{b \in V} \sum_{c \in V} \sum_{d \in V} {}^1T_{c,i} Y^{1,*}_{a,\epsilon} Z^*_{\epsilon,\gamma} Y^{3,*}_{b,\gamma} Y^{4,*}_{j,\gamma} {}^2D^{a,i,b,j} {}^2T_{b,j,d,k} V_{a,c,k,d} \quad (3535)$$

$$\tau^6_{\gamma,\delta,w} = \sum_{\epsilon \in A} Z_{\gamma,\epsilon} \tau^5_{\epsilon,\delta,w} \quad (2r_D r_T^3) \quad (3524)$$

Factorized expression

$$\tau^0_{\gamma,\alpha} = \sum_{a \in V} W^4_{a,\alpha} Y^3_{a,\gamma} \quad (2r_T r_V N_v) \quad (3536)$$

$${}^2R^2_{i,\gamma} \leftarrow - \sum_{\delta \in A} \sum_{w \in D} \frac{1}{2} {}^2D^2_{i,w} Y^2_{i,\delta} \tau^0_{\delta,\gamma,w} \tau^6_{\delta,\gamma,w} \quad (4r_D r_T^2 N_o) \quad (3525)$$

$$\tau^1_{\gamma,\alpha} = \sum_{i \in O} W^3_{i,\alpha} Y^4_{i,\gamma} \quad (2r_T r_V N_o) \quad (3537)$$

Raw expression

$${}^2R^2_{i,\epsilon} \leftarrow - \sum_{\gamma \in A} \sum_{j \in O} \sum_{k \in O} \sum_{a \in V} \sum_{b \in V} \sum_{c \in V} \frac{1}{2} {}^1T_{c,j} Y^{1,*}_{a,\epsilon} Z^*_{\epsilon,\gamma} Y^{3,*}_{b,\gamma} Y^{4,*}_{j,\gamma} f_{k,c} {}^2D^{a,i,b,j} {}^2T_{b,k,a,i} \quad (3526)$$

$$\tau^2_{\gamma,\alpha} = \sum_{\beta \in B} X_{\alpha,\beta} \tau^0_{\gamma,\beta} \tau^1_{\gamma,\beta} \quad (3r_T r_V^2) \quad (3538)$$

$$\tau^3_{\gamma,\alpha} = \sum_{\delta \in A} Z_{\gamma,\delta} \tau^2_{\delta,\alpha} \quad (2r_T^2 r_V) \quad (3539)$$

Factorized expression

$$\tau^0_{\gamma,\delta,w} = \sum_{a \in V} {}^2D^1_{a,w} Y^3_{a,\gamma} Y^{1,*}_{a,\delta} \quad (3r_D r_T^2 N_v) \quad (3527)$$

$$\tau^4_{\gamma,\delta,w} = \sum_{a \in V} {}^2D^3_{a,w} Y^1_{a,\gamma} Y^{3,*}_{a,\delta} \quad (3r_D r_T^2 N_v) \quad (3540)$$

$$\tau^1_{\gamma,\delta,w} = \sum_{a \in V} {}^2D^3_{a,w} Y^1_{a,\gamma} Y^{3,*}_{a,\delta} \quad (3r_D r_T^2 N_v) \quad (3528)$$

$$\tau^5_{\gamma,\delta,w} = \sum_{i \in O} {}^2D^4_{i,w} Y^2_{i,\gamma} Y^{4,*}_{i,\delta} \quad (3r_D r_T^2 N_o) \quad (3541)$$

$$\tau^2_{i,j} = \sum_{a \in V} {}^1T_{a,i} f_{j,a} \quad (2N_o^2 N_v) \quad (3529)$$

$$\tau^6_{\gamma,\delta,w} = \sum_{\epsilon \in A} Z^*_{\delta,\epsilon} \tau^4_{\gamma,\epsilon,w} \tau^5_{\gamma,\epsilon,w} \quad (3r_D r_T^3) \quad (3542)$$

$$\tau^3_{\gamma,i} = \sum_{j \in O} Y^2_{j,\gamma} \tau^2_{i,j} \quad (2r_T N_o^2) \quad (3530)$$

$$\tau^7_{\gamma,\alpha,w} = \sum_{\delta \in A} \tau^3_{\delta,\alpha} \tau^6_{\delta,\gamma,w} \quad (2r_D r_T^2 r_V) \quad (3543)$$

$$\tau^4_{\gamma,\delta,w} = \sum_{i \in O} {}^2D^4_{i,w} Y^{4,*}_{i,\delta} \tau^3_{\gamma,i} \quad (3r_D r_T^2 N_o) \quad (3531)$$

$$\tau^8_{\gamma,w,i} = \sum_{a \in V} {}^2D^1_{a,w} {}^1T_{a,i} Y^{1,*}_{a,\gamma} \quad (3r_D r_T N_o N_v) \quad (3544)$$

$$\tau^5_{\gamma,\delta,w} = \sum_{\epsilon \in A} Z^*_{\delta,\epsilon} \tau^1_{\gamma,\epsilon,w} \tau^4_{\gamma,\epsilon,w} \quad (3r_D r_T^3) \quad (3532)$$

$$\tau^9_{\gamma,\alpha,w} = \sum_{i \in O} W^1_{i,\alpha} \tau^8_{\gamma,w,i} \quad (2r_D r_T r_V N_o) \quad (3545)$$

$$\tau_{\gamma,w,i}^{10} = \sum_{\alpha \in B} W_{i,\alpha}^2 \tau_{\gamma,\alpha,w}^7 \tau_{\gamma,\alpha,w}^9 \quad (3r_D r_T r_V N_o) \quad (3546)$$

$$\tau_{\gamma,w,i}^{10} = \sum_{\alpha \in B} W_{i,\alpha}^2 \tau_{\gamma,\alpha,w}^7 \tau_{\gamma,\alpha,w}^9 \quad (3r_D r_T r_V N_o) \quad (3559)$$

$${}^2R_{i,\gamma}^2 \leftarrow - \sum_{w \in D} {}^2D_{i,w}^2 \tau_{\gamma,w,i}^{10} \quad (2r_D r_T N_o) \quad (3547)$$

$${}^2R_{i,\gamma}^2 \leftarrow - \sum_{w \in D} {}^2D_{i,w}^2 \tau_{\gamma,w,i}^{10} \quad (2r_D r_T N_o) \quad (3560)$$

Raw expression

$${}^2R_{i,\epsilon}^2 \leftarrow \sum_{\gamma \in A} \sum_{j \in O} \sum_{k \in O} \sum_{a \in V} \sum_{b \in V} \sum_{c \in V} \sum_{d \in V} {}^1T_{c,i} Y_{a,\epsilon}^{1,*} Z_{\epsilon,\gamma}^* Y_{b,\gamma}^{3,*} Y_{j,\gamma}^{4,*} {}^2D_{a,i,b,j} {}^2T_{d,k,b,j} V_{a,c,k,d} \quad (3548)$$

Raw expression

$${}^2R_{i,\epsilon}^2 \leftarrow \sum_{\gamma \in A} \sum_{j \in O} \sum_{k \in O} \sum_{a \in V} \sum_{b \in V} \sum_{c \in V} \sum_{d \in V} {}^1T_{c,j} Y_{a,\epsilon}^{1,*} Z_{\epsilon,\gamma}^* Y_{b,\gamma}^{3,*} Y_{j,\gamma}^{4,*} {}^2D_{a,i,b,j} {}^2T_{a,i,d,k} V_{b,c,k,d} \quad (3561)$$

Factorized expression

$$\tau_{\gamma,\delta,w}^0 = \sum_{a \in V} {}^2D_{a,w}^3 Y_{a,\gamma}^3 Y_{a,\delta}^{3,*} \quad (3r_D r_T^2 N_v) \quad (3549)$$

$$\tau_{\gamma,\delta,w}^0 = \sum_{a \in V} {}^2D_{a,w}^1 Y_{a,\gamma}^1 Y_{a,\delta}^{1,*} \quad (3r_D r_T^2 N_v) \quad (3562)$$

$$\tau_{\gamma,\delta,w}^1 = \sum_{i \in O} {}^2D_{i,w}^4 Y_{i,\gamma}^4 Y_{i,\delta}^{4,*} \quad (3r_D r_T^2 N_o) \quad (3550)$$

$$\tau_{\gamma,\alpha}^1 = \sum_{a \in V} W_{a,\alpha}^2 Y_{a,\gamma}^3 \quad (2r_T r_V N_v) \quad (3563)$$

$$\tau_{\gamma,\delta,w}^2 = \sum_{\epsilon \in A} Z_{\delta,\epsilon}^* \tau_{\gamma,\epsilon,w}^0 \tau_{\gamma,\epsilon,w}^1 \quad (3r_D r_T^3) \quad (3551)$$

$$\tau_{\gamma,\alpha}^2 = \sum_{i \in O} W_{i,\alpha}^1 Y_{i,\gamma}^4 \quad (2r_T r_V N_o) \quad (3564)$$

$$\tau_{\gamma,\alpha}^3 = \sum_{a \in V} W_{a,\alpha}^4 Y_{a,\gamma}^1 \quad (2r_T r_V N_v) \quad (3552)$$

$$\tau_{\gamma,\alpha}^3 = \sum_{\beta \in B} X_{\beta,\alpha} \tau_{\gamma,\beta}^1 \tau_{\gamma,\beta}^2 \quad (3r_T r_V^2) \quad (3565)$$

$$\tau_{\gamma,\alpha}^4 = \sum_{i \in O} W_{i,\alpha}^3 Y_{i,\gamma}^2 \quad (2r_T r_V N_o) \quad (3553)$$

$$\tau_{\gamma,\alpha}^4 = \sum_{\delta \in A} Z_{\gamma,\delta} \tau_{\delta,\alpha}^3 \quad (2r_T^2 r_V) \quad (3566)$$

$$\tau_{\gamma,\alpha}^5 = \sum_{\beta \in B} X_{\alpha,\beta} \tau_{\gamma,\beta}^3 \tau_{\gamma,\beta}^4 \quad (3r_T r_V^2) \quad (3554)$$

$$\tau_{\gamma,w,i}^5 = \sum_{a \in V} {}^2D_{a,w}^3 {}^1T_{a,i} Y_{a,\gamma}^{3,*} \quad (3r_D r_T N_o N_v) \quad (3567)$$

$$\tau_{\gamma,\alpha}^6 = \sum_{\delta \in A} Z_{\delta,\gamma} \tau_{\delta,\alpha}^5 \quad (2r_T^2 r_V) \quad (3555)$$

$$\tau_{\gamma,\alpha,w}^6 = \sum_{i \in O} W_{i,\alpha}^3 \tau_{\gamma,w,i}^5 \quad (2r_D r_T r_V N_o) \quad (3568)$$

$$\tau_{\gamma,\alpha,w}^7 = \sum_{\delta \in A} \tau_{\delta,\alpha}^6 \tau_{\delta,\gamma,w}^2 \quad (2r_D r_T^2 r_V) \quad (3556)$$

$$\tau_{\gamma,\alpha,w}^7 = \sum_{i \in O} {}^2D_{i,w}^4 W_{i,\alpha}^4 Y_{i,\gamma}^{4,*} \quad (3r_D r_T r_V N_o) \quad (3569)$$

$$\tau_{\gamma,w,i}^8 = \sum_{a \in V} {}^2D_{a,w}^1 {}^1T_{a,i} Y_{a,\gamma}^{1,*} \quad (3r_D r_T N_o N_v) \quad (3557)$$

$$\tau_{\gamma,\delta,w}^8 = \sum_{\alpha \in B} \tau_{\gamma,\alpha}^4 \tau_{\delta,\alpha,w}^6 \tau_{\delta,\alpha,w}^7 \quad (3r_D r_T^2 r_V) \quad (3570)$$

$$\tau_{\gamma,\alpha,w}^9 = \sum_{i \in O} W_{i,\alpha}^1 \tau_{\gamma,w,i}^8 \quad (2r_D r_T r_V N_o) \quad (3558)$$

$$\tau_{\gamma,\delta,w}^9 = \sum_{\epsilon \in A} Z_{\delta,\epsilon}^* \tau_{\gamma,\epsilon,w}^8 \quad (2r_D r_T^3) \quad (3571)$$

Raw expression

$${}^2R^2_{i,\gamma} \leftarrow - \sum_{\delta \in A} \sum_{w \in D} {}^2D^2_{i,w} Y^2_{i,\delta} \tau^0_{\delta,\gamma,w} \tau^9_{\delta,\gamma,w} \quad (4r_D r_T^2 N_o) \quad {}^2R^2_{i,\epsilon} \leftarrow \sum_{\gamma \in A} \sum_{j \in O} \sum_{k \in O} \sum_{a \in V} \sum_{b \in V} \sum_{c \in V} \sum_{d \in V} {}^1T_{c,k} Y^{1,*}_{a,\epsilon} Z^*_{\epsilon,\gamma} Y^{3,*}_{b,\gamma} Y^{4,*}_{j,\gamma} {}^2D^{a,i,b,j} {}^2T_{a,i,d,j} V_{b,d,k,c} \quad (3572) \quad (3585)$$

Raw expression

$${}^2R^2_{i,\epsilon} \leftarrow \sum_{\gamma \in A} \sum_{j \in O} \sum_{k \in O} \sum_{a \in V} \sum_{b \in V} \sum_{c \in V} \sum_{d \in V} {}^1T_{c,j} Y^{1,*}_{a,\epsilon} Z^*_{\epsilon,\gamma} Y^{3,*}_{b,\gamma} Y^{4,*}_{j,\gamma} {}^2D^{a,i,b,j} {}^2T_{d,k,a,i} V_{b,c,k,d} \quad (3573)$$

Factorized expression

$$\tau^0_{\gamma,\delta,w} = \sum_{a \in V} {}^2D^1_{a,w} Y^3_{a,\gamma} Y^{1,*}_{a,\delta} \quad (3r_D r_T^2 N_v) \quad (3574)$$

$$\tau^1_{\gamma,\alpha} = \sum_{a \in V} W^2_{a,\alpha} Y^1_{a,\gamma} \quad (2r_T r_V N_v) \quad (3575)$$

$$\tau^2_{\gamma,\alpha} = \sum_{i \in O} W^1_{i,\alpha} Y^2_{i,\gamma} \quad (2r_T r_V N_o) \quad (3576)$$

$$\tau^3_{\gamma,\alpha} = \sum_{\beta \in B} X_{\beta,\alpha} \tau^1_{\gamma,\beta} \tau^2_{\gamma,\beta} \quad (3r_T r_V^2) \quad (3577)$$

$$\tau^4_{\gamma,\alpha} = \sum_{\delta \in A} Z_{\delta,\gamma} \tau^3_{\delta,\alpha} \quad (2r_T^2 r_V) \quad (3578)$$

$$\tau^5_{\gamma,w,i} = \sum_{a \in V} {}^2D^3_{a,w} {}^1T_{a,i} Y^{3,*}_{a,\gamma} \quad (3r_D r_T N_o N_v) \quad (3579)$$

$$\tau^6_{\gamma,\alpha,w} = \sum_{i \in O} W^3_{i,\alpha} \tau^5_{\gamma,w,i} \quad (2r_D r_T r_V N_o) \quad (3580)$$

$$\tau^7_{\gamma,\alpha,w} = \sum_{i \in O} {}^2D^4_{i,w} W^4_{i,\alpha} Y^{4,*}_{i,\gamma} \quad (3r_D r_T r_V N_o) \quad (3581)$$

$$\tau^8_{\gamma,\delta,w} = \sum_{\alpha \in B} \tau^4_{\gamma,\alpha} \tau^6_{\delta,\alpha,w} \tau^7_{\delta,\alpha,w} \quad (3r_D r_T^2 r_V) \quad (3582)$$

$$\tau^9_{\gamma,\delta,w} = \sum_{\epsilon \in A} Z^*_{\delta,\epsilon} \tau^8_{\gamma,\epsilon,w} \quad (2r_D r_T^3) \quad (3583)$$

$${}^2R^2_{i,\gamma} \leftarrow - \sum_{\delta \in A} \sum_{w \in D} {}^2D^2_{i,w} Y^4_{i,\delta} \tau^0_{\delta,\gamma,w} \tau^9_{\delta,\gamma,w} \quad (4r_D r_T^2 N_o) \quad (3584)$$

Factorized expression

$$\tau^0_{\gamma,\delta,w} = \sum_{a \in V} {}^2D^1_{a,w} Y^1_{a,\gamma} Y^{1,*}_{a,\delta} \quad (3r_D r_T^2 N_v) \quad (3586)$$

$$\tau^1_{\gamma,\delta,w} = \sum_{a \in V} {}^2D^3_{a,w} Y^3_{a,\gamma} Y^{3,*}_{a,\delta} \quad (3r_D r_T^2 N_v) \quad (3587)$$

$$\tau^2_{\alpha,i} = \sum_{a \in V} {}^1T_{a,i} W^2_{a,\alpha} \quad (2r_V N_o N_v) \quad (3588)$$

$$\tau^3_{\alpha} = \sum_{i \in O} W^1_{i,\alpha} \tau^2_{\alpha,i} \quad (2r_V N_o) \quad (3589)$$

$$\tau^4_{\alpha} = \sum_{\beta \in B} \tau^3_{\beta} X_{\beta,\alpha} \quad (2r_V^2) \quad (3590)$$

$$\tau^5_{i,j} = \sum_{\alpha \in B} \tau^4_{\alpha} W^3_{i,\alpha} W^4_{j,\alpha} \quad (3r_V N_o^2) \quad (3591)$$

$$\tau^6_{\gamma,i} = \sum_{j \in O} Y^4_{j,\gamma} \tau^5_{j,i} \quad (2r_T N_o^2) \quad (3592)$$

$$\tau^7_{\gamma,\delta,w} = \sum_{i \in O} {}^2D^4_{i,w} Y^{4,*}_{i,\delta} \tau^6_{\gamma,i} \quad (3r_D r_T^2 N_o) \quad (3593)$$

$$\tau^8_{\gamma,\delta,w} = \sum_{\epsilon \in A} Z^*_{\delta,\epsilon} \tau^1_{\gamma,\epsilon,w} \tau^7_{\gamma,\epsilon,w} \quad (3r_D r_T^3) \quad (3594)$$

$$\tau^9_{\gamma,\delta,w} = \sum_{\epsilon \in A} Z_{\gamma,\epsilon} \tau^8_{\epsilon,\delta,w} \quad (2r_D r_T^3) \quad (3595)$$

$${}^2R^2_{i,\gamma} \leftarrow - \sum_{\delta \in A} \sum_{w \in D} {}^2D^2_{i,w} Y^2_{i,\delta} \tau^0_{\delta,\gamma,w} \tau^9_{\delta,\gamma,w} \quad (4r_D r_T^2 N_o) \quad (3596)$$

Raw expression

$${}^2R^2_{i,\epsilon} \leftarrow \sum_{\gamma \in A} \sum_{j \in O} \sum_{k \in O} \sum_{a \in V} \sum_{b \in V} \sum_{c \in V} \sum_{d \in V} {}^1T_{c,k} Y^{1,*}_{a,\epsilon} Z^*_{\epsilon,\gamma} Y^{3,*}_{b,\gamma} Y^{4,*}_{j,\gamma} {}^2D^{a,i,b,j} {}^2T_{b,j,d,i} V_{a,d,k,c} \quad (3597)$$

Factorized expression

$$\tau_{\gamma,\delta,w}^0 = \sum_{a \in V} {}^2D_{a,w}^1 Y_{a,\gamma}^3 Y_{a,\delta}^{1,*} \quad (3r_D r_T^2 N_v) \quad (3598)$$

$$\tau_{\gamma,\delta,w}^1 = \sum_{a \in V} {}^2D_{a,w}^3 Y_{a,\gamma}^1 Y_{a,\delta}^{3,*} \quad (3r_D r_T^2 N_v) \quad (3599)$$

$$\tau_{\alpha,i}^2 = \sum_{a \in V} {}^1T_{a,i} W_{a,\alpha}^2 \quad (2r_V N_o N_v) \quad (3600)$$

$$\tau_{\alpha}^3 = \sum_{i \in O} W_{i,\alpha}^1 \tau_{\alpha,i}^2 \quad (2r_V N_o) \quad (3601)$$

$$\tau_{\alpha}^4 = \sum_{\beta \in B} \tau_{\beta}^3 X_{\beta,\alpha} \quad (2r_V^2) \quad (3602)$$

$$\tau_{i,j}^5 = \sum_{\alpha \in B} \tau_{\alpha}^4 W_{i,\alpha}^3 W_{j,\alpha}^4 \quad (3r_V N_o^2) \quad (3603)$$

$$\tau_{\gamma,i}^6 = \sum_{j \in O} Y_{j,\gamma}^2 \tau_{j,i}^5 \quad (2r_T N_o^2) \quad (3604)$$

$$\tau_{\gamma,\delta,w}^7 = \sum_{i \in O} {}^2D_{i,w}^4 Y_{i,\delta}^{4,*} \tau_{\gamma,i}^6 \quad (3r_D r_T^2 N_o) \quad (3605)$$

$$\tau_{\gamma,\delta,w}^8 = \sum_{\epsilon \in A} Z_{\delta,\epsilon}^* \tau_{\gamma,\epsilon,w}^1 \tau_{\gamma,\epsilon,w}^7 \quad (3r_D r_T^3) \quad (3606)$$

$$\tau_{\gamma,\delta,w}^9 = \sum_{\epsilon \in A} Z_{\epsilon,\gamma} \tau_{\epsilon,\delta,w}^8 \quad (2r_D r_T^3) \quad (3607)$$

$${}^2R_{i,\gamma}^2 \leftarrow - \sum_{\delta \in A} \sum_{w \in D} {}^2D_{i,w}^2 Y_{i,\delta}^4 \tau_{\delta,\gamma,w}^0 \tau_{\delta,\gamma,w}^9 \quad (4r_D r_T^2 N_o) \quad (3608)$$

Raw expression

$${}^2R_{i,\epsilon}^2 \leftarrow \sum_{\gamma \in A} \sum_{j \in O} \sum_{k \in O} \sum_{a \in V} \sum_{b \in V} \sum_{c \in V} \sum_{d \in V} {}^1T_{c,k} Y_{a,\epsilon}^{1,*} Z_{\epsilon,\gamma}^* Y_{b,\gamma}^{3,*} Y_{j,\gamma}^{4,*} {}^2D_{a,i,b,j} {}^2T_{d,i,b,j} V_{a,d,k,c} \quad (3609)$$

Factorized expression

$$\tau_{\gamma,\delta,w}^0 = \sum_{a \in V} {}^2D_{a,w}^1 Y_{a,\gamma}^1 Y_{a,\delta}^{1,*} \quad (3r_D r_T^2 N_v) \quad (3610)$$

$$\tau_{\gamma,\delta,w}^1 = \sum_{a \in V} {}^2D_{a,w}^3 Y_{a,\gamma}^3 Y_{a,\delta}^{3,*} \quad (3r_D r_T^2 N_v) \quad (3611)$$

$$\tau_{\gamma,\delta,w}^2 = \sum_{i \in O} {}^2D_{i,w}^4 Y_{i,\gamma}^4 Y_{i,\delta}^{4,*} \quad (3r_D r_T^2 N_o) \quad (3612)$$

$$\tau_{\gamma,\delta,w}^3 = \sum_{\epsilon \in A} Z_{\delta,\epsilon}^* \tau_{\gamma,\epsilon,w}^1 \tau_{\gamma,\epsilon,w}^2 \quad (3r_D r_T^3) \quad (3613)$$

$$\tau_{\gamma,\delta,w}^4 = \sum_{\epsilon \in A} Z_{\gamma,\epsilon} \tau_{\epsilon,\delta,w}^3 \quad (2r_D r_T^3) \quad (3614)$$

$$\tau_{\alpha,i}^5 = \sum_{a \in V} {}^1T_{a,i} W_{a,\alpha}^4 \quad (2r_V N_o N_v) \quad (3615)$$

$$\tau_{\alpha}^6 = \sum_{i \in O} W_{i,\alpha}^3 \tau_{\alpha,i}^5 \quad (2r_V N_o) \quad (3616)$$

$$\tau_{\alpha}^7 = \sum_{\beta \in B} \tau_{\beta}^6 X_{\alpha,\beta} \quad (2r_V^2) \quad (3617)$$

$$\tau_{i,j}^8 = \sum_{\alpha \in B} \tau_{\alpha}^7 W_{i,\alpha}^1 W_{j,\alpha}^2 \quad (3r_V N_o^2) \quad (3618)$$

$$\tau_{\gamma,i}^9 = \sum_{j \in O} Y_{j,\gamma}^2 \tau_{j,i}^8 \quad (2r_T N_o^2) \quad (3619)$$

$${}^2R_{i,\gamma}^2 \leftarrow - \sum_{\delta \in A} \sum_{w \in D} {}^2D_{i,w}^2 \tau_{\delta,i}^9 \tau_{\delta,\gamma,w}^0 \tau_{\delta,\gamma,w}^4 \quad (4r_D r_T^2 N_o) \quad (3620)$$

Raw expression

$${}^2R_{i,\epsilon}^2 \leftarrow \sum_{\gamma \in A} \sum_{j \in O} \sum_{k \in O} \sum_{a \in V} \sum_{b \in V} \sum_{c \in V} \sum_{d \in V} {}^1T_{c,k} Y_{a,\epsilon}^{1,*} Z_{\epsilon,\gamma}^* Y_{b,\gamma}^{3,*} Y_{j,\gamma}^{4,*} {}^2D_{a,i,b,j} {}^2T_{d,j,a,i} V_{b,d,k,c} \quad (3621)$$

Factorized expression

$$\tau_{\gamma,\delta,w}^0 = \sum_{a \in V} {}^2D_{a,w}^3 Y_{a,\gamma}^1 Y_{a,\delta}^{3,*} \quad (3r_D r_T^2 N_v) \quad (3622)$$

$$\tau_{\gamma,\delta,w}^1 = \sum_{i \in O} {}^2D_{i,w}^4 Y_{i,\gamma}^2 Y_{i,\delta}^{4,*} \quad (3r_D r_T^2 N_o) \quad (3623)$$

$$\tau_{\gamma,\delta,w}^2 = \sum_{\epsilon \in A} Z_{\delta,\epsilon}^* \tau_{\gamma,\epsilon,w}^0 \tau_{\gamma,\epsilon,w}^1 \quad (3r_D r_T^3) \quad (3624)$$

$$\tau_{\alpha,i,j}^3 = \sum_{\beta \in B} X_{\alpha,\beta} W_{i,\beta}^3 W_{j,\beta}^4 \quad (3r_V^2 N_o^2) \quad (3637)$$

$$\tau_{\gamma,\delta,w}^3 = \sum_{\epsilon \in A} Z_{\epsilon,\gamma} \tau_{\epsilon,\delta,w}^2 \quad (2r_D r_T^3) \quad (3625)$$

$$\tau_{\gamma,\alpha,i}^4 = \sum_{j \in O} Y_{j,\gamma}^2 \tau_{\alpha,j,i}^3 \quad (2r_T r_V N_o^2) \quad (3638)$$

$$\tau_{\gamma,\delta,w}^4 = \sum_{a \in V} {}^2D_{a,w}^1 Y_{a,\gamma}^3 Y_{a,\delta}^{1,*} \quad (3r_D r_T^2 N_v) \quad (3626)$$

$$\tau_{\gamma,\delta,\alpha,w}^5 = \sum_{i \in O} {}^2D_{i,w}^4 Y_{i,\delta}^{4,*} \tau_{\gamma,\delta,w}^2 \tau_{\gamma,\alpha,i}^4 \quad (4r_D r_T^2 r_V N_o) \quad (3639)$$

$$\tau_{\alpha,i}^5 = \sum_{a \in V} {}^1T_{a,i} W_{a,\alpha}^4 \quad (2r_V N_o N_v) \quad (3627)$$

$$\tau_{\gamma,\alpha,w,i}^6 = \sum_{\delta \in A} \tau_{\delta,\alpha,i}^1 \tau_{\delta,\gamma,\alpha,w}^5 \quad (2r_D r_T^2 r_V N_o) \quad (3640)$$

$$\tau_{\alpha}^6 = \sum_{i \in O} W_{i,\alpha}^3 \tau_{\alpha,i}^5 \quad (2r_V N_o) \quad (3628)$$

$$\tau_{\gamma,w,i,j}^7 = \sum_{\alpha \in B} W_{i,\alpha}^1 \tau_{\gamma,\alpha,w,j}^6 \quad (2r_D r_T r_V N_o^2) \quad (3641)$$

$$\tau_{\alpha}^7 = \sum_{\beta \in B} \tau_{\beta}^6 X_{\alpha,\beta} \quad (2r_V^2) \quad (3629)$$

$$\tau_{\gamma,w,i,j}^8 = \sum_{\delta \in A} Z_{\gamma,\delta}^* \tau_{\delta,w,i,j}^7 \quad (2r_D r_T^2 N_o^2) \quad (3642)$$

$$\tau_{i,j}^8 = \sum_{\alpha \in B} \tau_{\alpha}^7 W_{i,\alpha}^1 W_{j,\alpha}^2 \quad (3r_V N_o^2) \quad (3630)$$

$$\tau_{\gamma,w,i}^9 = \sum_{a \in V} {}^2D_{a,w}^1 {}^1T_{a,i} Y_{a,\gamma}^{1,*} \quad (3r_D r_T N_o N_v) \quad (3643)$$

$$\tau_{\gamma,i}^9 = \sum_{j \in O} Y_{j,\gamma}^4 \tau_{j,i}^8 \quad (2r_T N_o^2) \quad (3631)$$

$$\tau_{\gamma,w,i}^{10} = \sum_{j \in O} \tau_{\gamma,w,j}^9 \tau_{\gamma,w,j,i}^8 \quad (2r_D r_T N_o^2) \quad (3644)$$

$${}^2R_{i,\gamma}^2 \leftarrow - \sum_{\delta \in A} \sum_{w \in D} {}^2D_{i,w}^2 \tau_{\delta,i}^9 \tau_{\delta,\gamma,w}^3 \tau_{\delta,\gamma,w}^4 \quad (4r_D r_T^2 N_o) \quad (3632)$$

$${}^2R_{i,\gamma}^2 \leftarrow \sum_{w \in D} \frac{1}{2} {}^2D_{i,w}^2 \tau_{\gamma,w,i}^{10} \quad (2r_D r_T N_o) \quad (3645)$$

Raw expression

$${}^2R_{i,\epsilon}^2 \leftarrow - \sum_{\gamma \in A} \sum_{j \in O} \sum_{k \in O} \sum_{a \in V} \sum_{b \in V} \sum_{c \in V} \sum_{d \in V} \frac{1}{2} {}^1T_{a,k} Y_{a,\epsilon}^{1,*} Z_{\epsilon,\gamma}^* Y_{b,\gamma}^{3,*} Y_{j,\gamma}^{4,*} {}^2D_{a,i,b,j} {}^2T_{c,i,d,j} V_{b,d,k,c} \quad (3633)$$

Raw expression

$${}^2R_{i,\epsilon}^2 \leftarrow - \sum_{\gamma \in A} \sum_{j \in O} \sum_{k \in O} \sum_{a \in V} \sum_{b \in V} \sum_{c \in V} \sum_{d \in V} \frac{1}{2} {}^1T_{a,k} Y_{a,\epsilon}^{1,*} Z_{\epsilon,\gamma}^* Y_{b,\gamma}^{3,*} Y_{j,\gamma}^{4,*} {}^2D_{a,i,b,j} {}^2T_{c,j,d,i} V_{b,c,k,d} \quad (3646)$$

Factorized expression

$$\tau_{\gamma,\alpha}^0 = \sum_{a \in V} W_{a,\alpha}^2 Y_{a,\gamma}^3 \quad (2r_T r_V N_v) \quad (3634)$$

$$\tau_{\gamma,\delta,w}^0 = \sum_{a \in V} {}^2D_{a,w}^3 Y_{a,\gamma}^3 Y_{a,\delta}^{3,*} \quad (3r_D r_T^2 N_v) \quad (3647)$$

$$\tau_{\gamma,\alpha,i}^1 = \sum_{\delta \in A} Z_{\gamma,\delta} Y_{i,\delta}^4 \tau_{\delta,\alpha}^0 \quad (3r_T^2 r_V N_o) \quad (3635)$$

$$\tau_{\alpha,i,j}^1 = \sum_{\beta \in B} X_{\alpha,\beta} W_{i,\beta}^3 W_{j,\beta}^4 \quad (3r_V^2 N_o^2) \quad (3648)$$

$$\tau_{\gamma,\delta,w}^2 = \sum_{a \in V} {}^2D_{a,w}^3 Y_{a,\gamma}^1 Y_{a,\delta}^{3,*} \quad (3r_D r_T^2 N_v) \quad (3636)$$

$$\tau_{\gamma,\alpha,i}^2 = \sum_{j \in O} Y_{j,\gamma}^4 \tau_{\alpha,j,i}^1 \quad (2r_T r_V N_o^2) \quad (3649)$$



$$\tau^3_{\gamma,\delta,\alpha,w} = \sum_{i \in O} {}^2D^4_{i,w} Y^{4,*}_{i,\delta} \tau^0_{\gamma,\delta,w} \tau^2_{\gamma,\alpha,i} \quad (4r_D r_T^2 r_V N_o) \quad (3650)$$

$$\tau^4_{\gamma,\alpha} = \sum_{a \in V} W^2_{a,\alpha} Y^1_{a,\gamma} \quad (2r_T r_V N_v) \quad (3651)$$

$$\tau^5_{\gamma,\alpha,i} = \sum_{\delta \in A} Y^2_{i,\delta} Z_{\delta,\gamma} \tau^4_{\delta,\alpha} \quad (3r_T^2 r_V N_o) \quad (3652)$$

$$\tau^6_{\gamma,\alpha,w,i} = \sum_{\delta \in A} \tau^5_{\delta,\alpha,i} \tau^3_{\delta,\gamma,\alpha,w} \quad (2r_D r_T^2 r_V N_o) \quad (3653)$$

$$\tau^7_{\gamma,w,i,j} = \sum_{\alpha \in B} W^1_{i,\alpha} \tau^6_{\gamma,\alpha,w,j} \quad (2r_D r_T r_V N_o^2) \quad (3654)$$

$$\tau^8_{\gamma,w,i,j} = \sum_{\delta \in A} Z^*_{\gamma,\delta} \tau^7_{\delta,w,i,j} \quad (2r_D r_T^2 N_o^2) \quad (3655)$$

$$\tau^9_{\gamma,w,i} = \sum_{a \in V} {}^2D^1_{a,w} {}^1T_{a,i} Y^{1,*}_{a,\gamma} \quad (3r_D r_T N_o N_v) \quad (3656)$$

$$\tau^{10}_{\gamma,w,i} = \sum_{j \in O} \tau^9_{\gamma,w,j} \tau^8_{\gamma,w,j,i} \quad (2r_D r_T N_o^2) \quad (3657)$$

$${}^2R^2_{i,\gamma} \leftarrow \sum_{w \in D} \frac{1}{2} {}^2D^2_{i,w} \tau^{10}_{\gamma,w,i} \quad (2r_D r_T N_o) \quad (3658)$$

Raw expression

$${}^2R^2_{i,\epsilon} \leftarrow - \sum_{\gamma \in A} \sum_{j \in O} \sum_{k \in O} \sum_{a \in V} \sum_{b \in V} \sum_{c \in V} \sum_{d \in V} \frac{1}{2} {}^1T_{b,k} Y^{1,*}_{a,\epsilon} Z^*_{\epsilon,\gamma} Y^{3,*}_{b,\gamma} Y^{4,*}_{j,\gamma} {}^2D^{a,i,b,j} {}^2T_{c,i,d,j} V_{a,c,k,d} \quad (3659)$$

Factorized expression

$$\tau^0_{\gamma,\delta,w} = \sum_{a \in V} {}^2D^3_{a,w} Y^1_{a,\gamma} Y^{3,*}_{a,\delta} \quad (3r_D r_T^2 N_v) \quad (3660)$$

$$\tau^1_{\gamma,\alpha} = \sum_{i \in O} W^3_{i,\alpha} Y^2_{i,\gamma} \quad (2r_T r_V N_o) \quad (3661)$$

$$\tau^2_{\gamma,\alpha} = \sum_{a \in V} W^4_{a,\alpha} Y^3_{a,\gamma} \quad (2r_T r_V N_v) \quad (3662)$$

$$\tau^3_{\gamma,\alpha,i} = \sum_{\delta \in A} Z_{\gamma,\delta} Y^4_{i,\delta} \tau^2_{\delta,\alpha} \quad (3r_T^2 r_V N_o) \quad (3663)$$

$$\tau^4_{\gamma,\alpha,w} = \sum_{\delta \in A} \sum_{i \in O} {}^2D^4_{i,w} Y^{4,*}_{i,\gamma} \tau^1_{\delta,\alpha} \tau^0_{\delta,\gamma,w} \tau^3_{\delta,\alpha,i} \quad (5r_D r_T^2 r_V N_o) \quad (3664)$$

$$\tau^5_{\gamma,\alpha,w} = \sum_{\beta \in B} X_{\alpha,\beta} \tau^4_{\gamma,\beta,w} \quad (2r_D r_T r_V^2) \quad (3665)$$

$$\tau^6_{\gamma,\alpha,w} = \sum_{\delta \in A} Z^*_{\gamma,\delta} \tau^5_{\delta,\alpha,w} \quad (2r_D r_T^2 r_V) \quad (3666)$$

$$\tau^7_{\gamma,w,i} = \sum_{a \in V} {}^2D^1_{a,w} {}^1T_{a,i} Y^{1,*}_{a,\gamma} \quad (3r_D r_T N_o N_v) \quad (3667)$$

$$\tau^8_{\gamma,\alpha,w} = \sum_{i \in O} W^1_{i,\alpha} \tau^7_{\gamma,w,i} \quad (2r_D r_T r_V N_o) \quad (3668)$$

$$\tau^9_{\gamma,w,i} = \sum_{\alpha \in B} W^2_{i,\alpha} \tau^6_{\gamma,\alpha,w} \tau^8_{\gamma,\alpha,w} \quad (3r_D r_T r_V N_o) \quad (3669)$$

$${}^2R^2_{i,\gamma} \leftarrow \sum_{w \in D} \frac{1}{2} {}^2D^2_{i,w} \tau^9_{\gamma,w,i} \quad (2r_D r_T N_o) \quad (3670)$$

Raw expression

$${}^2R^2_{i,\epsilon} \leftarrow - \sum_{\gamma \in A} \sum_{j \in O} \sum_{k \in O} \sum_{a \in V} \sum_{b \in V} \sum_{c \in V} \sum_{d \in V} \frac{1}{2} {}^1T_{b,k} Y^{1,*}_{a,\epsilon} Z^*_{\epsilon,\gamma} Y^{3,*}_{b,\gamma} Y^{4,*}_{j,\gamma} {}^2D^{a,i,b,j} {}^2T_{c,j,d,i} V_{a,d,k,c} \quad (3671)$$

Factorized expression

$$\tau^0_{\gamma,\delta,w} = \sum_{a \in V} {}^2D^3_{a,w} Y^3_{a,\gamma} Y^{3,*}_{a,\delta} \quad (3r_D r_T^2 N_v) \quad (3672)$$

$$\tau^1_{\gamma,\alpha} = \sum_{a \in V} W^4_{a,\alpha} Y^1_{a,\gamma} \quad (2r_T r_V N_v) \quad (3673)$$

$$\tau^2_{\gamma,\alpha,i} = \sum_{\delta \in A} Y^2_{i,\delta} Z_{\delta,\gamma} \tau^1_{\delta,\alpha} \quad (3r_T^2 r_V N_o) \quad (3674)$$

$$\tau^3_{\gamma,\alpha} = \sum_{i \in O} W^3_{i,\alpha} Y^4_{i,\gamma} \quad (2r_T r_V N_o) \quad (3675)$$

$$\tau^4_{\gamma,\alpha,w} = \sum_{\delta \in A} \sum_{i \in O} {}^2D^4_{i,w} Y^{4,*}_{i,\gamma} \tau^3_{\delta,\alpha} \tau^0_{\delta,\gamma,w} \tau^2_{\delta,\alpha,i} \quad (5r_D r_T^2 r_V N_o) \quad (3676)$$

$$\tau^5_{\gamma,\alpha,w} = \sum_{\beta \in B} X_{\alpha,\beta} \tau^4_{\gamma,\beta,w} \quad (2r_D r_T r_V^2) \quad (3677)$$

$$\tau^6_{\gamma,\alpha,w} = \sum_{\delta \in A} Z^*_{\gamma,\delta} \tau^5_{\delta,\alpha,w} \quad (2r_D r_T^2 r_V) \quad (3678)$$

$$\tau^7_{\gamma,w,i} = \sum_{a \in V} {}^2D^1_{a,w} {}^1T_{a,i} Y^{1,*}_{a,\gamma} \quad (3r_D r_T N_o N_v) \quad (3679)$$

$$\tau^8_{\gamma,\alpha,w} = \sum_{i \in O} W^1_{i,\alpha} \tau^7_{\gamma,w,i} \quad (2r_D r_T r_V N_o) \quad (3680)$$

$$\tau^9_{\gamma,w,i} = \sum_{\alpha \in B} W^2_{i,\alpha} \tau^6_{\gamma,\alpha,w} \tau^8_{\gamma,\alpha,w} \quad (3r_D r_T r_V N_o) \quad (3681)$$

$${}^2R^2_{i,\gamma} \leftarrow \sum_{w \in D} \frac{1}{2} {}^2D^2_{i,w} \tau^9_{\gamma,w,i} \quad (2r_D r_T N_o) \quad (3682)$$

Raw expression

$${}^2R^2_{i,\epsilon} \leftarrow - \sum_{\gamma \in A} \sum_{j \in O} \sum_{k \in O} \sum_{a \in V} \sum_{b \in V} \sum_{c \in V} \sum_{d \in V} \frac{1}{2} {}^1T_{c,i} Y^{1,*}_{a,\epsilon} Z^*_{\epsilon,\gamma} Y^{3,*}_{b,\gamma} Y^{4,*}_{j,\gamma} {}^2D^{a,i,b,j} {}^2T_{a,k,d,j} V_{b,d,k,c} \quad (3683)$$

Factorized expression

$$\tau^0_{\alpha,i,j} = \sum_{\beta \in B} W^1_{i,\beta} W^2_{j,\beta} X_{\beta,\alpha} \quad (3r_V^2 N_o^2) \quad (3684)$$

$$\tau^1_{\gamma,\alpha,i} = \sum_{j \in O} Y^4_{j,\gamma} \tau^0_{\alpha,j,i} \quad (2r_T r_V N_o^2) \quad (3685)$$

$$\tau^2_{\gamma,\alpha} = \sum_{a \in V} W^4_{a,\alpha} Y^3_{a,\gamma} \quad (2r_T r_V N_v) \quad (3686)$$

$$\tau^3_{\gamma,i,j} = \sum_{\alpha \in B} W^3_{j,\alpha} \tau^2_{\gamma,\alpha} \tau^1_{\gamma,\alpha,i} \quad (3r_T r_V N_o^2) \quad (3687)$$

$$\tau^4_{\gamma,i,j} = \sum_{\delta \in A} Z_{\gamma,\delta} \tau^3_{\delta,i,j} \quad (2r_T^2 N_o^2) \quad (3688)$$

$$\tau^6_{\gamma,\delta,w} = \sum_{i \in O} {}^2D^4_{i,w} Y^2_{i,\gamma} Y^{4,*}_{i,\delta} \quad (3r_D r_T^2 N_o) \quad (3690)$$

$$\tau^7_{\gamma,\delta,w} = \sum_{\epsilon \in A} Z^*_{\delta,\epsilon} \tau^5_{\gamma,\epsilon,w} \tau^6_{\gamma,\epsilon,w} \quad (3r_D r_T^3) \quad (3691)$$

$$\tau^8_{\gamma,w,i,j} = \sum_{\delta \in A} \tau^4_{\delta,i,j} \tau^7_{\delta,\gamma,w} \quad (2r_D r_T^2 N_o^2) \quad (3692)$$

$$\tau^9_{\gamma,w,i} = \sum_{a \in V} {}^2D^1_{a,w} {}^1T_{a,i} Y^{1,*}_{a,\gamma} \quad (3r_D r_T N_o N_v) \quad (3693)$$

$$\tau^{10}_{\gamma,w,i} = \sum_{j \in O} \tau^9_{\gamma,w,j} \tau^8_{\gamma,w,i,j} \quad (2r_D r_T N_o^2) \quad (3694)$$

$${}^2R^2_{i,\gamma} \leftarrow \sum_{w \in D} \frac{1}{2} {}^2D^2_{i,w} \tau^{10}_{\gamma,w,i} \quad (2r_D r_T N_o) \quad (3695)$$

Raw expression

$${}^2R^2_{i,\epsilon} \leftarrow - \sum_{\gamma \in A} \sum_{j \in O} \sum_{k \in O} \sum_{a \in V} \sum_{b \in V} \sum_{c \in V} \sum_{d \in V} \frac{1}{2} {}^1T_{c,i} Y^{1,*}_{a,\epsilon} Z^*_{\epsilon,\gamma} Y^{3,*}_{b,\gamma} Y^{4,*}_{j,\gamma} {}^2D^{a,i,b,j} {}^2T_{b,j,d,k} V_{a,d,k,c} \quad (3696)$$

Factorized expression

$$\tau^0_{\alpha,i,j} = \sum_{\beta \in B} W^1_{i,\beta} W^2_{j,\beta} X_{\beta,\alpha} \quad (3r_V^2 N_o^2) \quad (3697)$$

$$\tau^1_{\gamma,\alpha,i} = \sum_{j \in O} Y^2_{j,\gamma} \tau^0_{\alpha,j,i} \quad (2r_T r_V N_o^2) \quad (3698)$$

$$\tau^2_{\gamma,\alpha} = \sum_{a \in V} W^4_{a,\alpha} Y^1_{a,\gamma} \quad (2r_T r_V N_v) \quad (3699)$$

$$\tau^3_{\gamma,i,j} = \sum_{\alpha \in B} W^3_{j,\alpha} \tau^2_{\gamma,\alpha} \tau^1_{\gamma,\alpha,i} \quad (3r_T r_V N_o^2) \quad (3700)$$

$$\tau^4_{\gamma,i,j} = \sum_{\delta \in A} Z_{\delta,\gamma} \tau^3_{\delta,i,j} \quad (2r_T^2 N_o^2) \quad (3701)$$

$$\tau^5_{\gamma,\delta,w} = \sum_{a \in V} {}^2D^3_{a,w} Y^3_{a,\gamma} Y^{3,*}_{a,\delta} \quad (3r_D r_T^2 N_v) \quad (3702)$$

$$\tau^6_{\gamma,\delta,w} = \sum_{i \in O} {}^2D^4_{i,w} Y^4_{i,\gamma} Y^{4,*}_{i,\delta} \quad (3r_D r_T^2 N_o) \quad (3703)$$

$$\tau^7_{\gamma,\delta,w} = \sum_{\epsilon \in A} Z^*_{\delta,\epsilon} \tau^5_{\gamma,\epsilon,w} \tau^6_{\gamma,\epsilon,w} \quad (3r_D r_T^3) \quad (3704)$$

$$\tau^8_{\gamma,w,i,j} = \sum_{\delta \in A} \tau^4_{\delta,i,j} \tau^7_{\delta,\gamma,w} \quad (2r_D r_T^2 N_o^2) \quad (3705)$$

$$\tau^9_{\gamma,w,i} = \sum_{a \in V} {}^2D^1_{a,w} {}^1T_{a,i} Y^{1,*}_{a,\gamma} \quad (3r_D r_T N_o N_v) \quad (3706)$$

$$\tau^{10}_{\gamma,w,i} = \sum_{j \in O} \tau^9_{\gamma,w,j} \tau^8_{\gamma,w,i,j} \quad (2r_D r_T N_o^2) \quad (3707)$$

$${}^2R^2_{i,\gamma} \leftarrow \sum_{w \in D} \frac{1}{2} {}^2D^2_{i,w} \tau^{10}_{\gamma,w,i} \quad (2r_D r_T N_o) \quad (3708)$$

Raw expression

$${}^2R^2_{i,\epsilon} \leftarrow - \sum_{\gamma \in A} \sum_{j \in O} \sum_{k \in O} \sum_{a \in V} \sum_{b \in V} \sum_{c \in V} \sum_{d \in V} \frac{1}{2} {}^1T_{c,i} Y^{1,*}_{a,\epsilon} Z^*_{\epsilon,\gamma} Y^{3,*}_{b,\gamma} Y^{4,*}_{j,\gamma} {}^2D^{a,i,b,j} {}^2T_{b,k,d,j} V_{a,c,k,d} \quad (3709)$$

Factorized expression

$$\tau^0_{\gamma,\delta,w} = \sum_{a \in V} {}^2D^1_{a,w} Y^1_{a,\gamma} Y^{1,*}_{a,\delta} \quad (3r_D r_T^2 N_v) \quad (3710)$$

$$\tau^1_{\gamma,w,i} = \sum_{a \in V} {}^2D^3_{a,w} {}^1T_{a,i} Y^{3,*}_{a,\gamma} \quad (3r_D r_T N_o N_v) \quad (3711)$$

$$\tau^2_{\gamma,\alpha} = \sum_{a \in V} W^2_{a,\alpha} Y^3_{a,\gamma} \quad (2r_T r_V N_v) \quad (3712)$$

$$\tau^3_{\alpha,i,j} = \sum_{\beta \in B} X_{\alpha,\beta} W^3_{i,\beta} W^4_{j,\beta} \quad (3r_V^2 N_o^2) \quad (3713)$$

$$\tau^4_{\gamma,\alpha,i} = \sum_{j \in O} Y^4_{j,\gamma} \tau^3_{\alpha,j,i} \quad (2r_T r_V N_o^2) \quad (3714)$$

$$\tau^5_{\gamma,i,j} = \sum_{\alpha \in B} W^1_{i,\alpha} \tau^2_{\gamma,\alpha} \tau^4_{\gamma,\alpha,j} \quad (3r_T r_V N_o^2) \quad (3715)$$

$$\tau^6_{\gamma,i,j} = \sum_{\delta \in A} Z_{\gamma,\delta} \tau^5_{\delta,i,j} \quad (2r_T^2 N_o^2) \quad (3716)$$

$$\tau^7_{\gamma,\delta,w} = \sum_{i \in O} \sum_{j \in O} {}^2D^4_{i,w} Y^{4,*}_{i,\delta} \tau^1_{\delta,w,j} \tau^6_{\gamma,j,i} \quad (4r_D r_T^2 N_o^2) \quad (3717)$$

$$\tau^8_{\gamma,\delta,w} = \sum_{\epsilon \in A} Z^*_{\delta,\epsilon} \tau^7_{\gamma,\epsilon,w} \quad (2r_D r_T^3) \quad (3718)$$

$${}^2R^2_{i,\gamma} \leftarrow \sum_{\delta \in A} \sum_{w \in D} \frac{1}{2} {}^2D^2_{i,w} Y^2_{i,\delta} \tau^0_{\delta,\gamma,w} \tau^8_{\delta,\gamma,w} \quad (4r_D r_T^2 N_o) \quad (3719)$$

Raw expression

$${}^2R^2_{i,\epsilon} \leftarrow - \sum_{\gamma \in A} \sum_{j \in O} \sum_{k \in O} \sum_{a \in V} \sum_{b \in V} \sum_{c \in V} \sum_{d \in V} \frac{1}{2} {}^1T_{c,i} Y^{1,*}_{a,\epsilon} Z^*_{\epsilon,\gamma} Y^{3,*}_{b,\gamma} Y^{4,*}_{j,\gamma} {}^2D^{a,i,b,j} {}^2T_{d,j,a,k} V_{b,d,k,c} \quad (3720)$$

Factorized expression

$$\tau^0_{\gamma,\delta,w} = \sum_{a \in V} {}^2D^1_{a,w} Y^3_{a,\gamma} Y^{1,*}_{a,\delta} \quad (3r_D r_T^2 N_v) \quad (3721)$$

$$\tau^1_{\gamma,w,i} = \sum_{a \in V} {}^2D^3_{a,w} {}^1T_{a,i} Y^{3,*}_{a,\gamma} \quad (3r_D r_T N_o N_v) \quad (3722)$$

$$\tau^2_{\gamma,\alpha} = \sum_{a \in V} W^2_{a,\alpha} Y^1_{a,\gamma} \quad (2r_T r_V N_v) \quad (3723)$$

$$\tau^3_{\alpha,i,j} = \sum_{\beta \in B} X_{\alpha,\beta} W^3_{i,\beta} W^4_{j,\beta} \quad (3r_V^2 N_o^2) \quad (3724)$$

$$\tau^4_{\gamma,\alpha,i} = \sum_{j \in O} Y^2_{j,\gamma} \tau^3_{\alpha,j,i} \quad (2r_T r_V N_o^2) \quad (3725)$$

$$\tau^5_{\gamma,i,j} = \sum_{\alpha \in B} W^1_{i,\alpha} \tau^2_{\gamma,\alpha} \tau^4_{\gamma,\alpha,j} \quad (3r_T r_V N_o^2) \quad (3726)$$

$$\tau^6_{\gamma,i,j} = \sum_{\delta \in A} Z_{\delta,\gamma} \tau^5_{\delta,i,j} \quad (2r_T^2 N_o^2) \quad (3727)$$

$$\tau_{\gamma,\delta,w}^7 = \sum_{i \in O} \sum_{j \in O} {}^2D_{i,w}^4 Y_{i,\delta}^{4,*} \tau_{\delta,w,j}^1 \tau_{\gamma,j,i}^6 \quad (4r_D r_T^2 N_o^2) \quad (3728)$$

$$\tau_{\gamma,\delta,w}^8 = \sum_{\epsilon \in A} Z_{\delta,\epsilon}^* \tau_{\gamma,\epsilon,w}^7 \quad (2r_D r_T^3) \quad (3729)$$

$${}^2R_{i,\gamma}^2 \leftarrow \sum_{\delta \in A} \sum_{w \in D} \frac{1}{2} {}^2D_{i,w}^2 Y_{i,\delta}^4 \tau_{\delta,\gamma,w}^0 \tau_{\delta,\gamma,w}^8 \quad (4r_D r_T^2 N_o) \quad (3730)$$

Raw expression

$${}^2R_{i,\epsilon}^2 \leftarrow - \sum_{\gamma \in A} \sum_{j \in O} \sum_{k \in O} \sum_{a \in V} \sum_{b \in V} \sum_{c \in V} \sum_{d \in V} \frac{1}{2} {}^1T_{c,i} Y_{a,\epsilon}^{1,*} Z_{\epsilon,\gamma}^* Y_{b,\gamma}^{3,*} Y_{j,\gamma}^{4,*} {}^2D_{a,i,b,j} {}^2T_{d,j,b,k} V_{a,c,k,d} \quad (3731)$$

Factorized expression

$$\tau_{\gamma,\delta,w}^0 = \sum_{a \in V} {}^2D_{a,w}^1 Y_{a,\gamma}^1 Y_{a,\delta}^{1,*} \quad (3r_D r_T^2 N_v) \quad (3732)$$

$$\tau_{\gamma,\alpha}^1 = \sum_{i \in O} W_{i,\alpha}^1 Y_{i,\gamma}^2 \quad (2r_T r_V N_o) \quad (3733)$$

$$\tau_{\gamma,\alpha}^2 = \sum_{a \in V} W_{a,\alpha}^2 Y_{a,\gamma}^3 \quad (2r_T r_V N_v) \quad (3734)$$

$$\tau_{\gamma,\alpha,i}^3 = \sum_{\delta \in A} Z_{\gamma,\delta} Y_{i,\delta}^4 \tau_{\delta,\alpha}^2 \quad (3r_T^2 r_V N_o) \quad (3735)$$

$$\tau_{\gamma,w,i}^4 = \sum_{a \in V} {}^2D_{a,w}^3 {}^1T_{a,i} Y_{a,\gamma}^{3,*} \quad (3r_D r_T N_o N_v) \quad (3736)$$

$$\tau_{\gamma,\alpha,w}^5 = \sum_{i \in O} W_{i,\alpha}^3 \tau_{\gamma,w,i}^4 \quad (2r_D r_T r_V N_o) \quad (3737)$$

$$\tau_{\gamma,\alpha,w}^6 = \sum_{i \in O} {}^2D_{i,w}^4 W_{i,\alpha}^4 Y_{i,\gamma}^{4,*} \quad (3r_D r_T r_V N_o) \quad (3738)$$

$$\tau_{\gamma,\alpha,w}^7 = \sum_{\beta \in B} X_{\alpha,\beta} \tau_{\gamma,\beta,w}^5 \tau_{\gamma,\beta,w}^6 \quad (3r_D r_T r_V^2) \quad (3739)$$

$$\tau_{\gamma,\alpha,w}^8 = \sum_{\delta \in A} Z_{\gamma,\delta}^* \tau_{\delta,\alpha,w}^7 \quad (2r_D r_T^2 r_V) \quad (3740)$$

$$\tau_{\gamma,\delta,w,i}^9 = \sum_{\alpha \in B} \tau_{\gamma,\alpha}^1 \tau_{\gamma,\alpha,i}^3 \tau_{\delta,\alpha,w}^8 \quad (3r_D r_T^2 r_V N_o) \quad (3741)$$

$$\tau_{\gamma,w,i}^{10} = \sum_{\delta \in A} \tau_{\delta,\gamma,w}^0 \tau_{\delta,\gamma,w,i}^9 \quad (2r_D r_T^2 N_o) \quad (3742)$$

$${}^2R_{i,\gamma}^2 \leftarrow \sum_{w \in D} \frac{1}{2} {}^2D_{i,w}^2 \tau_{\gamma,w,i}^{10} \quad (2r_D r_T N_o) \quad (3743)$$

Raw expression

$${}^2R_{i,\epsilon}^2 \leftarrow - \sum_{\gamma \in A} \sum_{j \in O} \sum_{k \in O} \sum_{a \in V} \sum_{b \in V} \sum_{c \in V} \sum_{d \in V} \frac{1}{2} {}^1T_{c,i} Y_{a,\epsilon}^{1,*} Z_{\epsilon,\gamma}^* Y_{b,\gamma}^{3,*} Y_{j,\gamma}^{4,*} {}^2D_{a,i,b,j} {}^2T_{d,k,b,j} V_{a,d,k,c} \quad (3744)$$

Factorized expression

$$\tau_{\gamma,\alpha}^0 = \sum_{a \in V} W_{a,\alpha}^2 Y_{a,\gamma}^1 \quad (2r_T r_V N_v) \quad (3745)$$

$$\tau_{\gamma,\alpha,i}^1 = \sum_{\delta \in A} Y_{i,\delta}^2 Z_{\delta,\gamma} \tau_{\delta,\alpha}^0 \quad (3r_T^2 r_V N_o) \quad (3746)$$

$$\tau_{\gamma,\alpha}^2 = \sum_{i \in O} W_{i,\alpha}^1 Y_{i,\gamma}^4 \quad (2r_T r_V N_o) \quad (3747)$$

$$\tau_{\gamma,w,i}^3 = \sum_{a \in V} {}^2D_{a,w}^3 {}^1T_{a,i} Y_{a,\gamma}^{3,*} \quad (3r_D r_T N_o N_v) \quad (3748)$$

$$\tau_{\gamma,\alpha,w}^4 = \sum_{i \in O} W_{i,\alpha}^3 \tau_{\gamma,w,i}^3 \quad (2r_D r_T r_V N_o) \quad (3749)$$

$$\tau_{\gamma,\alpha,w}^5 = \sum_{i \in O} {}^2D_{i,w}^4 W_{i,\alpha}^4 Y_{i,\gamma}^{4,*} \quad (3r_D r_T r_V N_o) \quad (3750)$$

$$\tau_{\gamma,\alpha,w}^6 = \sum_{\beta \in B} X_{\alpha,\beta} \tau_{\gamma,\beta,w}^4 \tau_{\gamma,\beta,w}^5 \quad (3r_D r_T r_V^2) \quad (3751)$$

$$\tau_{\gamma,\alpha,w}^7 = \sum_{\delta \in A} Z_{\gamma,\delta}^* \tau_{\delta,\alpha,w}^6 \quad (2r_D r_T^2 r_V) \quad (3752)$$

$$\tau_{\gamma,\delta,w,i}^8 = \sum_{\alpha \in B} \tau_{\gamma,\alpha}^2 \tau_{\gamma,\alpha,i}^1 \tau_{\delta,\alpha,w}^7 \quad (3r_D r_T^2 r_V N_o) \quad (3753)$$

$$\tau_{\gamma,\delta,w}^9 = \sum_{a \in V} {}^2D_{a,w}^1 Y_{a,\gamma}^3 Y_{a,\delta}^{1,*} \quad (3r_D r_T^2 N_v) \quad (3754)$$

$$\tau_{\gamma,w,i}^{10} = \sum_{\delta \in A} \tau_{\delta,\gamma,w}^9 \tau_{\delta,\gamma,w,i}^8 \quad (2r_D r_T^2 N_o) \quad (3755)$$

$${}^2R_{i,\gamma}^2 \leftarrow \sum_{w \in D} \frac{1}{2} {}^2D_{i,w}^2 \tau_{\gamma,w,i}^{10} \quad (2r_D r_T N_o) \quad (3756)$$

Raw expression

$${}^2R_{i,\epsilon}^2 \leftarrow - \sum_{\gamma \in A} \sum_{j \in O} \sum_{k \in O} \sum_{a \in V} \sum_{b \in V} \sum_{c \in V} \sum_{d \in V} \frac{1}{2} {}^1T_{c,j} Y_{a,\epsilon}^{1,*} Z_{\epsilon,\gamma}^* Y_{b,\gamma}^{3,*} Y_{j,\gamma}^{4,*} {}^2D_{a,i,b,j} {}^2T_{a,i,d,k} V_{b,d,k,c} \quad (3757)$$

Factorized expression

$$\tau_{\gamma,\delta,w}^0 = \sum_{a \in V} {}^2D_{a,w}^1 Y_{a,\gamma}^1 Y_{a,\delta}^{1,*} \quad (3r_D r_T^2 N_v) \quad (3758)$$

$$\tau_{\alpha,i,j}^1 = \sum_{\beta \in B} W_{i,\beta}^1 W_{j,\beta}^2 X_{\beta,\alpha} \quad (3r_V^2 N_o^2) \quad (3759)$$

$$\tau_{\gamma,\alpha,i}^2 = \sum_{j \in O} Y_{j,\gamma}^2 \tau_{\alpha,j,i}^1 \quad (2r_T r_V N_o^2) \quad (3760)$$

$$\tau_{\gamma,w,i}^3 = \sum_{a \in V} {}^2D_{a,w}^3 T_{a,i}^1 Y_{a,\gamma}^{3,*} \quad (3r_D r_T N_o N_v) \quad (3761)$$

$$\tau_{\gamma,w,i,j}^4 = \sum_{\delta \in A} {}^2D_{i,w}^4 Z_{\gamma,\delta}^* Y_{i,\delta}^{4,*} \tau_{\delta,w,j}^3 \quad (4r_D r_T^2 N_o^2) \quad (3762)$$

$$\tau_{\gamma,\alpha,w,i}^5 = \sum_{j \in O} W_{j,\alpha}^3 \tau_{\gamma,w,i,j}^4 \quad (2r_D r_T r_V N_o^2) \quad (3763)$$

$$\tau_{\gamma,\alpha}^6 = \sum_{a \in V} W_{a,\alpha}^4 Y_{a,\gamma}^3 \quad (2r_T r_V N_v) \quad (3764)$$

$$\tau_{\gamma,\alpha,i}^7 = \sum_{\delta \in A} Z_{\gamma,\delta} Y_{i,\delta}^4 \tau_{\delta,\alpha}^6 \quad (3r_T^2 r_V N_o) \quad (3765)$$

$$\tau_{\gamma,\delta,\alpha,w}^8 = \sum_{i \in O} \tau_{\gamma,\alpha,i}^7 \tau_{\delta,\alpha,w,i}^5 \quad (2r_D r_T^2 r_V N_o) \quad (3766)$$

$$\tau_{\gamma,\delta,w,i}^9 = \sum_{\alpha \in B} \tau_{\gamma,\alpha,i}^2 \tau_{\gamma,\delta,\alpha,w}^8 \quad (2r_D r_T^2 r_V N_o) \quad (3767)$$

$$\tau_{\gamma,w,i}^{10} = \sum_{\delta \in A} \tau_{\delta,\gamma,w}^0 \tau_{\delta,\gamma,w,i}^9 \quad (2r_D r_T^2 N_o) \quad (3768)$$

$${}^2R_{i,\gamma}^2 \leftarrow \sum_{w \in D} \frac{1}{2} {}^2D_{i,w}^2 \tau_{\gamma,w,i}^{10} \quad (2r_D r_T N_o) \quad (3769)$$

Raw expression

$${}^2R_{i,\epsilon}^2 \leftarrow - \sum_{\gamma \in A} \sum_{j \in O} \sum_{k \in O} \sum_{a \in V} \sum_{b \in V} \sum_{c \in V} \sum_{d \in V} \frac{1}{2} {}^1T_{c,j} Y_{a,\epsilon}^{1,*} Z_{\epsilon,\gamma}^* Y_{b,\gamma}^{3,*} Y_{j,\gamma}^{4,*} {}^2D_{a,i,b,j} {}^2T_{a,k,d,i} V_{b,c,k,d} \quad (3770)$$

Factorized expression

$$\tau_{\alpha,i,j}^0 = \sum_{\beta \in B} W_{i,\beta}^1 W_{j,\beta}^2 X_{\beta,\alpha} \quad (3r_V^2 N_o^2) \quad (3771)$$

$$\tau_{\gamma,\alpha,i}^1 = \sum_{j \in O} Y_{j,\gamma}^4 \tau_{\alpha,j,i}^0 \quad (2r_T r_V N_o^2) \quad (3772)$$

$$\tau_{\gamma,w,i}^2 = \sum_{a \in V} {}^2D_{a,w}^3 T_{a,i}^1 Y_{a,\gamma}^{3,*} \quad (3r_D r_T N_o N_v) \quad (3773)$$

$$\tau_{\gamma,w,i,j}^3 = \sum_{\delta \in A} {}^2D_{i,w}^4 Z_{\gamma,\delta}^* Y_{i,\delta}^{4,*} \tau_{\delta,w,j}^2 \quad (4r_D r_T^2 N_o^2) \quad (3774)$$

$$\tau_{\gamma,\alpha,w,i}^4 = \sum_{j \in O} W_{j,\alpha}^3 \tau_{\gamma,w,i,j}^3 \quad (2r_D r_T r_V N_o^2) \quad (3775)$$

$$\tau_{\gamma,\alpha}^5 = \sum_{a \in V} W_{a,\alpha}^4 Y_{a,\gamma}^1 \quad (2r_T r_V N_v) \quad (3776)$$

$$\tau_{\gamma,\alpha,i}^6 = \sum_{\delta \in A} Y_{i,\delta}^2 Z_{\delta,\gamma} \tau_{\delta,\alpha}^5 \quad (3r_T^2 r_V N_o) \quad (3777)$$

$$\tau_{\gamma,\delta,\alpha,w}^7 = \sum_{i \in O} \tau_{\gamma,\alpha,i}^6 \tau_{\delta,\alpha,w,i}^4 \quad (2r_D r_T^2 r_V N_o) \quad (3778)$$

$$\tau_{\gamma,\delta,w,i}^8 = \sum_{\alpha \in B} \tau_{\gamma,\alpha,i}^1 \tau_{\gamma,\delta,\alpha,w}^7 \quad (2r_D r_T^2 r_V N_o) \quad (3779)$$

$$\tau_{\gamma,\delta,w}^9 = \sum_{a \in V} {}^2D_{a,w}^1 Y_{a,\gamma}^3 Y_{a,\delta}^{1,*} \quad (3r_D r_T^2 N_v) \quad (3780)$$

$$\tau_{\gamma,w,i}^{10} = \sum_{\delta \in A} \tau_{\delta,\gamma,w}^9 \tau_{\delta,\gamma,w,i}^8 \quad (2r_D r_T^2 N_o) \quad (3781)$$

$${}^2R_{i,\gamma}^2 \leftarrow \sum_{w \in D} \frac{1}{2} {}^2D_{i,w}^2 \tau_{\gamma,w,i}^{10} \quad (2r_D r_T N_o) \quad (3782)$$

Raw expression

$${}^2R_{i,\epsilon}^2 \leftarrow - \sum_{\gamma \in A} \sum_{j \in O} \sum_{k \in O} \sum_{a \in V} \sum_{b \in V} \sum_{c \in V} \sum_{d \in V} \frac{1}{2} {}^1T_{c,j} Y_{a,\epsilon}^{1,*} Z_{\epsilon,\gamma}^* Y_{b,\gamma}^{3,*} Y_{j,\gamma}^{4,*} {}^2D_{a,i,b,j} {}^2T_{b,k,d,i} V_{a,d,k,c} \quad (3783)$$

Factorized expression

$$\tau_{\gamma,\delta,w}^0 = \sum_{a \in V} {}^2D_{a,w}^1 Y_{a,\gamma}^1 Y_{a,\delta}^{1,*} \quad (3r_D r_T^2 N_v) \quad (3784)$$

$$\tau_{\gamma,\alpha,w}^1 = \sum_{i \in O} {}^2D_{i,w}^4 W_{i,\alpha}^4 Y_{i,\gamma}^{4,*} \quad (3r_D r_T r_V N_o) \quad (3785)$$

$$\tau_{\gamma,\delta,w}^2 = \sum_{a \in V} {}^2D_{a,w}^3 Y_{a,\gamma}^3 Y_{a,\delta}^{3,*} \quad (3r_D r_T^2 N_v) \quad (3786)$$

$$\tau_{\gamma,\delta,w,i}^3 = \sum_{\epsilon \in A} Z_{\gamma,\epsilon} Y_{i,\epsilon}^4 \tau_{\epsilon,\delta,w}^2 \quad (3r_D r_T^3 N_o) \quad (3787)$$

$$\tau_{\gamma,\delta,\alpha,w}^4 = \sum_{i \in O} W_{i,\alpha}^3 \tau_{\delta,\alpha,w}^1 \tau_{\gamma,\delta,w,i}^3 \quad (3r_D r_T^2 r_V N_o) \quad (3788)$$

$$\tau_{\alpha,i}^5 = \sum_{a \in V} {}^1T_{a,i} W_{a,\alpha}^2 \quad (2r_V N_o N_v) \quad (3789)$$

$$\tau_{\alpha,i,j}^6 = \sum_{\beta \in B} W_{j,\beta}^1 X_{\beta,\alpha} \tau_{\beta,i}^5 \quad (3r_V^2 N_o^2) \quad (3790)$$

$$\tau_{\gamma,\alpha,i}^7 = \sum_{j \in O} Y_{j,\gamma}^2 \tau_{\alpha,i,j}^6 \quad (2r_T r_V N_o^2) \quad (3791)$$

$$\tau_{\gamma,\delta,w,i}^8 = \sum_{\alpha \in B} \tau_{\gamma,\alpha,i}^7 \tau_{\gamma,\delta,\alpha,w}^4 \quad (2r_D r_T^2 r_V N_o) \quad (3792)$$

$$\tau_{\gamma,\delta,i}^9 = \sum_{\epsilon \in A} \sum_{w \in D} {}^2D_{i,w}^2 \tau_{\epsilon,\gamma,w}^0 \tau_{\epsilon,\delta,w,i}^8 \quad (3r_D r_T^3 N_o) \quad (3793)$$

$${}^2R_{i,\gamma}^2 \leftarrow \sum_{\delta \in A} \frac{1}{2} Z_{\gamma,\delta}^* \tau_{\gamma,\delta,i}^9 \quad (2r_T^2 N_o) \quad (3794)$$

Raw expression

$${}^2R_{i,\epsilon}^2 \leftarrow - \sum_{\gamma \in A} \sum_{j \in O} \sum_{k \in O} \sum_{a \in V} \sum_{b \in V} \sum_{c \in V} \sum_{d \in V} \frac{1}{2} {}^1T_{c,j} Y_{a,\epsilon}^{1,*} Z_{\epsilon,\gamma}^* Y_{b,\gamma}^{3,*} Y_{j,\gamma}^{4,*} {}^2D_{a,i,b,j} {}^2T_{d,i,a,k} V_{b,c,k,d} \quad (3795)$$

Factorized expression

$$\tau_{\gamma,\delta,w}^0 = \sum_{a \in V} {}^2D_{a,w}^1 Y_{a,\gamma}^3 Y_{a,\delta}^{1,*} \quad (3r_D r_T^2 N_v) \quad (3796)$$

$$\tau_{\gamma,\alpha,w}^1 = \sum_{i \in O} {}^2D_{i,w}^4 W_{i,\alpha}^4 Y_{i,\gamma}^{4,*} \quad (3r_D r_T r_V N_o) \quad (3797)$$

$$\tau_{\gamma,\delta,w}^2 = \sum_{a \in V} {}^2D_{a,w}^3 Y_{a,\gamma}^3 Y_{a,\delta}^{3,*} \quad (3r_D r_T^2 N_v) \quad (3798)$$

$$\tau_{\gamma,\delta,w,i}^3 = \sum_{\epsilon \in A} Y_{i,\epsilon}^2 Z_{\epsilon,\gamma} \tau_{\epsilon,\delta,w}^2 \quad (3r_D r_T^3 N_o) \quad (3799)$$

$$\tau_{\gamma,\delta,\alpha,w}^4 = \sum_{i \in O} W_{i,\alpha}^3 \tau_{\delta,\alpha,w}^1 \tau_{\gamma,\delta,w,i}^3 \quad (3r_D r_T^2 r_V N_o) \quad (3800)$$

$$\tau_{\alpha,i}^5 = \sum_{a \in V} {}^1T_{a,i} W_{a,\alpha}^2 \quad (2r_V N_o N_v) \quad (3801)$$

$$\tau_{\alpha,i,j}^6 = \sum_{\beta \in B} W_{j,\beta}^1 X_{\beta,\alpha} \tau_{\beta,i}^5 \quad (3r_V^2 N_o^2) \quad (3802)$$

$$\tau_{\gamma,\alpha,i}^7 = \sum_{j \in O} Y_{j,\gamma}^4 \tau_{\alpha,i,j}^6 \quad (2r_T r_V N_o^2) \quad (3803)$$

$$\tau_{\gamma,\delta,w,i}^8 = \sum_{\alpha \in B} \tau_{\gamma,\alpha,i}^7 \tau_{\gamma,\delta,\alpha,w}^4 \quad (2r_D r_T^2 r_V N_o) \quad (3804)$$

$$\tau^9_{\gamma,\delta,i} = \sum_{\epsilon \in A} \sum_{w \in D} {}^2D^2_{i,w} \tau^0_{\epsilon,\gamma,w} \tau^8_{\epsilon,\delta,w,i} \quad (3r_D r_T^3 N_o) \quad (3805)$$

$${}^2R^2_{i,\gamma} \leftarrow \sum_{\delta \in A} \frac{1}{2} Z^*_{\gamma,\delta} \tau^9_{\gamma,\delta,i} \quad (2r_T^2 N_o) \quad (3806)$$

Raw expression

$${}^2R^2_{i,\epsilon} \leftarrow - \sum_{\gamma \in A} \sum_{j \in O} \sum_{k \in O} \sum_{a \in V} \sum_{b \in V} \sum_{c \in V} \sum_{d \in V} \frac{1}{2} {}^1T_{c,j} Y^{1,*}_{a,\epsilon} Z^*_{\epsilon,\gamma} Y^{3,*}_{b,\gamma} Y^{4,*}_{j,\gamma} {}^2D^{a,i,b,j} {}^2T_{d,i,b,k} V_{a,d,k,c} \quad (3807)$$

Factorized expression

$$\tau^0_{\gamma,\delta,w} = \sum_{a \in V} {}^2D^1_{a,w} Y^1_{a,\gamma} Y^{1,*}_{a,\delta} \quad (3r_D r_T^2 N_v) \quad (3808)$$

$$\tau^1_{\alpha,i} = \sum_{a \in V} {}^1T_{a,i} W^4_{a,\alpha} \quad (2r_V N_o N_v) \quad (3809)$$

$$\tau^2_{\gamma,\alpha,w} = \sum_{i \in O} {}^2D^4_{i,w} Y^{4,*}_{i,\gamma} \tau^1_{\alpha,i} \quad (3r_D r_T r_V N_o) \quad (3810)$$

$$\tau^3_{\gamma,\delta,w} = \sum_{a \in V} {}^2D^3_{a,w} Y^3_{a,\gamma} Y^{3,*}_{a,\delta} \quad (3r_D r_T^2 N_v) \quad (3811)$$

$$\tau^4_{\gamma,\delta,w,i} = \sum_{\epsilon \in A} Z_{\gamma,\epsilon} Y^4_{i,\epsilon} \tau^3_{\epsilon,\delta,w} \quad (3r_D r_T^3 N_o) \quad (3812)$$

$$\tau^5_{\gamma,\delta,\alpha,w} = \sum_{i \in O} W^3_{i,\alpha} \tau^2_{\delta,\alpha,w} \tau^4_{\gamma,\delta,w,i} \quad (3r_D r_T^2 r_V N_o) \quad (3813)$$

$$\tau^6_{\alpha,i,j} = \sum_{\beta \in B} W^1_{i,\beta} W^2_{j,\beta} X_{\beta,\alpha} \quad (3r_V^2 N_o^2) \quad (3814)$$

$$\tau^7_{\gamma,\alpha,i} = \sum_{j \in O} Y^2_{j,\gamma} \tau^6_{\alpha,j,i} \quad (2r_T r_V N_o^2) \quad (3815)$$

$$\tau^8_{\gamma,\delta,w,i} = \sum_{\alpha \in B} \tau^7_{\gamma,\alpha,i} \tau^5_{\gamma,\delta,\alpha,w} \quad (2r_D r_T^2 r_V N_o) \quad (3816)$$

$$\tau^9_{\gamma,\delta,i} = \sum_{\epsilon \in A} \sum_{w \in D} {}^2D^2_{i,w} \tau^0_{\epsilon,\gamma,w} \tau^8_{\epsilon,\delta,w,i} \quad (3r_D r_T^3 N_o) \quad (3817)$$

$${}^2R^2_{i,\gamma} \leftarrow \sum_{\delta \in A} \frac{1}{2} Z^*_{\gamma,\delta} \tau^9_{\gamma,\delta,i} \quad (2r_T^2 N_o) \quad (3818)$$

Raw expression

$${}^2R^2_{i,\epsilon} \leftarrow - \sum_{\gamma \in A} \sum_{j \in O} \sum_{k \in O} \sum_{a \in V} \sum_{b \in V} \sum_{c \in V} \sum_{d \in V} \frac{1}{2} {}^1T_{c,j} Y^{1,*}_{a,\epsilon} Z^*_{\epsilon,\gamma} Y^{3,*}_{b,\gamma} Y^{4,*}_{j,\gamma} {}^2D^{a,i,b,j} {}^2T_{d,k,a,i} V_{b,d,k,c} \quad (3819)$$

Factorized expression

$$\tau^0_{\gamma,\delta,w} = \sum_{a \in V} {}^2D^1_{a,w} Y^3_{a,\gamma} Y^{1,*}_{a,\delta} \quad (3r_D r_T^2 N_v) \quad (3820)$$

$$\tau^1_{\alpha,i} = \sum_{a \in V} {}^1T_{a,i} W^4_{a,\alpha} \quad (2r_V N_o N_v) \quad (3821)$$

$$\tau^2_{\gamma,\alpha,w} = \sum_{i \in O} {}^2D^4_{i,w} Y^{4,*}_{i,\gamma} \tau^1_{\alpha,i} \quad (3r_D r_T r_V N_o) \quad (3822)$$

$$\tau^3_{\gamma,\delta,w} = \sum_{a \in V} {}^2D^3_{a,w} Y^1_{a,\gamma} Y^{3,*}_{a,\delta} \quad (3r_D r_T^2 N_v) \quad (3823)$$

$$\tau^4_{\gamma,\delta,w,i} = \sum_{\epsilon \in A} Y^2_{i,\epsilon} Z_{\epsilon,\gamma} \tau^3_{\epsilon,\delta,w} \quad (3r_D r_T^3 N_o) \quad (3824)$$

$$\tau^5_{\gamma,\delta,\alpha,w} = \sum_{i \in O} W^3_{i,\alpha} \tau^2_{\delta,\alpha,w} \tau^4_{\gamma,\delta,w,i} \quad (3r_D r_T^2 r_V N_o) \quad (3825)$$

$$\tau^6_{\alpha,i,j} = \sum_{\beta \in B} W^1_{i,\beta} W^2_{j,\beta} X_{\beta,\alpha} \quad (3r_V^2 N_o^2) \quad (3826)$$

$$\tau^7_{\gamma,\alpha,i} = \sum_{j \in O} Y^4_{j,\gamma} \tau^6_{\alpha,j,i} \quad (2r_T r_V N_o^2) \quad (3827)$$

$$\tau^8_{\gamma,\delta,w,i} = \sum_{\alpha \in B} \tau^7_{\gamma,\alpha,i} \tau^5_{\gamma,\delta,\alpha,w} \quad (2r_D r_T^2 r_V N_o) \quad (3828)$$

$$\tau^9_{\gamma,\delta,i} = \sum_{\epsilon \in A} \sum_{w \in D} {}^2D^2_{i,w} \tau^0_{\epsilon,\gamma,w} \tau^8_{\epsilon,\delta,w,i} \quad (3r_D r_T^3 N_o) \quad (3829)$$

$${}^2R^2_{i,\gamma} \leftarrow \sum_{\delta \in A} \frac{1}{2} Z^*_{\gamma,\delta} \tau^9_{\gamma,\delta,i} \quad (2r_T^2 N_o) \quad (3830)$$

Raw expression

$${}^2R^2_{i,\epsilon} \leftarrow - \sum_{\gamma \in A} \sum_{j \in O} \sum_{k \in O} \sum_{a \in V} \sum_{b \in V} \sum_{c \in V} \sum_{d \in V} \frac{1}{2} {}^1T_{c,k} Y^{1,*}_{a,\epsilon} Z^*_{\epsilon,\gamma} Y^{3,*}_{b,\gamma} Y^{4,*}_{j,\gamma} {}^2D^{a,i,b,j} {}^2T_{a,i,d,j} V_{b,c,k,d} \quad (3831)$$

Factorized expression

$$\tau^0_{\gamma,\delta,w} = \sum_{a \in V} {}^2D^1_{a,w} Y^1_{a,\gamma} Y^{1,*}_{a,\delta} \quad (3r_D r_T^2 N_v) \quad (3832)$$

$$\tau^1_{\gamma,\delta,w} = \sum_{a \in V} {}^2D^3_{a,w} Y^3_{a,\gamma} Y^{3,*}_{a,\delta} \quad (3r_D r_T^2 N_v) \quad (3833)$$

$$\tau^2_{\gamma,\delta,w} = \sum_{i \in O} {}^2D^4_{i,w} Y^4_{i,\gamma} Y^{4,*}_{i,\delta} \quad (3r_D r_T^2 N_o) \quad (3834)$$

$$\tau^3_{\gamma,\delta,w} = \sum_{\epsilon \in A} Z^*_{\delta,\epsilon} \tau^1_{\gamma,\epsilon,w} \tau^2_{\gamma,\epsilon,w} \quad (3r_D r_T^3) \quad (3835)$$

$$\tau^4_{\gamma,\delta,w} = \sum_{\epsilon \in A} Z_{\gamma,\epsilon} \tau^3_{\epsilon,\delta,w} \quad (2r_D r_T^3) \quad (3836)$$

$$\tau^5_{\alpha,i} = \sum_{a \in V} {}^1T_{a,i} W^4_{a,\alpha} \quad (2r_V N_o N_v) \quad (3837)$$

$$\tau^6_{\alpha,\beta} = \sum_{i \in O} W^1_{i,\alpha} \tau^5_{\beta,i} \quad (2r_V^2 N_o) \quad (3838)$$

$$\tau^7_{\alpha,i} = \sum_{\beta \in B} X_{\alpha,\beta} W^3_{i,\beta} \tau^6_{\alpha,\beta} \quad (3r_V^2 N_o) \quad (3839)$$

$$\tau^8_{i,j} = \sum_{\alpha \in B} W^2_{i,\alpha} \tau^7_{\alpha,j} \quad (2r_V N_o^2) \quad (3840)$$

$$\tau^9_{\gamma,i} = \sum_{j \in O} Y^2_{j,\gamma} \tau^8_{i,j} \quad (2r_T N_o^2) \quad (3841)$$

Raw expression

$${}^2R^2_{i,\epsilon} \leftarrow - \sum_{\gamma \in A} \sum_{j \in O} \sum_{k \in O} \sum_{a \in V} \sum_{b \in V} \sum_{c \in V} \sum_{d \in V} \frac{1}{2} {}^1T_{c,k} Y^{1,*}_{a,\epsilon} Z^*_{\epsilon,\gamma} Y^{3,*}_{b,\gamma} Y^{4,*}_{j,\gamma} {}^2D^{a,i,b,j} {}^2T_{b,j,d,i} V_{a,c,k,d} \quad (3842)$$

Raw expression

Factorized expression

$$\tau^0_{\gamma,\delta,w} = \sum_{a \in V} {}^2D^3_{a,w} Y^1_{a,\gamma} Y^{3,*}_{a,\delta} \quad (3r_D r_T^2 N_v) \quad (3844)$$

$$\tau^1_{\gamma,\delta,w} = \sum_{i \in O} {}^2D^4_{i,w} Y^2_{i,\gamma} Y^{4,*}_{i,\delta} \quad (3r_D r_T^2 N_o) \quad (3845)$$

$$\tau^2_{\gamma,\delta,w} = \sum_{\epsilon \in A} Z^*_{\delta,\epsilon} \tau^0_{\gamma,\epsilon,w} \tau^1_{\gamma,\epsilon,w} \quad (3r_D r_T^3) \quad (3846)$$

$$\tau^3_{\gamma,\delta,w} = \sum_{\epsilon \in A} Z_{\epsilon,\gamma} \tau^2_{\epsilon,\delta,w} \quad (2r_D r_T^3) \quad (3847)$$

$$\tau^4_{\gamma,\delta,w} = \sum_{a \in V} {}^2D^1_{a,w} Y^3_{a,\gamma} Y^{1,*}_{a,\delta} \quad (3r_D r_T^2 N_v) \quad (3848)$$

$$\tau^5_{\alpha,i} = \sum_{a \in V} {}^1T_{a,i} W^4_{a,\alpha} \quad (2r_V N_o N_v) \quad (3849)$$

$$\tau^6_{\alpha,\beta} = \sum_{i \in O} W^1_{i,\alpha} \tau^5_{\beta,i} \quad (2r_V^2 N_o) \quad (3850)$$

$$\tau^7_{\alpha,i} = \sum_{\beta \in B} X_{\alpha,\beta} W^3_{i,\beta} \tau^6_{\alpha,\beta} \quad (3r_V^2 N_o) \quad (3851)$$

$$\tau^8_{i,j} = \sum_{\alpha \in B} W^2_{i,\alpha} \tau^7_{\alpha,j} \quad (2r_V N_o^2) \quad (3852)$$

$$\tau^9_{\gamma,i} = \sum_{j \in O} Y^4_{j,\gamma} \tau^8_{i,j} \quad (2r_T N_o^2) \quad (3853)$$

$${}^2R^2_{i,\gamma} \leftarrow \sum_{\delta \in A} \sum_{w \in D} \frac{1}{2} {}^2D^2_{i,w} \tau^9_{\delta,i} \tau^3_{\delta,\gamma,w} \tau^4_{\delta,\gamma,w} \quad (4r_D r_T^2 N_o) \quad (3854)$$

Raw expression

$${}^2R^2_{i,\epsilon} \leftarrow - \sum_{\gamma \in A} \sum_{j \in O} \sum_{k \in O} \sum_{a \in V} \sum_{b \in V} \sum_{c \in V} \sum_{d \in V} \frac{1}{2} {}^1T_{c,k} Y^{1,*}_{a,\epsilon} Z^*_{\epsilon,\gamma} Y^{3,*}_{b,\gamma} Y^{4,*}_{j,\gamma} {}^2D^{a,i,b,j} {}^2T_{d,i,b,j} V_{a,c,k,d} \quad (3855)$$

Factorized expression

$$\tau^0_{\gamma,\delta,w} = \sum_{a \in V} {}^2D^1_{a,w} Y^1_{a,\gamma} Y^{1,*}_{a,\delta} \quad (3r_D r_T^2 N_v) \quad (3856)$$



$$\tau^1_{\gamma,\delta,w} = \sum_{a \in V} {}^2D^3_{a,w} Y^3_{a,\gamma} Y^{3,*}_{a,\delta} \quad (3r_D r_T^2 N_v) \quad (3857)$$

$$\tau^2_{\alpha,i} = \sum_{a \in V} {}^1T_{a,i} W^2_{a,\alpha} \quad (2r_V N_o N_v) \quad (3870)$$

$$\tau^2_{\alpha,i} = \sum_{a \in V} {}^1T_{a,i} W^2_{a,\alpha} \quad (2r_V N_o N_v) \quad (3858)$$

$$\tau^3_{\alpha,\beta} = \sum_{i \in O} W^3_{i,\beta} \tau^2_{\alpha,i} \quad (2r_V^2 N_o) \quad (3871)$$

$$\tau^3_{\alpha,\beta} = \sum_{i \in O} W^3_{i,\beta} \tau^2_{\alpha,i} \quad (2r_V^2 N_o) \quad (3859)$$

$$\tau^4_{\alpha,i} = \sum_{\beta \in B} X_{\alpha,\beta} W^4_{i,\beta} \tau^3_{\alpha,\beta} \quad (3r_V^2 N_o) \quad (3872)$$

$$\tau^4_{\alpha,i} = \sum_{\beta \in B} X_{\alpha,\beta} W^4_{i,\beta} \tau^3_{\alpha,\beta} \quad (3r_V^2 N_o) \quad (3860)$$

$$\tau^5_{i,j} = \sum_{\alpha \in B} W^1_{i,\alpha} \tau^4_{\alpha,j} \quad (2r_V N_o^2) \quad (3873)$$

$$\tau^5_{i,j} = \sum_{\alpha \in B} W^1_{i,\alpha} \tau^4_{\alpha,j} \quad (2r_V N_o^2) \quad (3861)$$

$$\tau^6_{\gamma,i} = \sum_{j \in O} Y^2_{j,\gamma} \tau^5_{j,i} \quad (2r_T N_o^2) \quad (3874)$$

$$\tau^6_{\gamma,i} = \sum_{j \in O} Y^4_{j,\gamma} \tau^5_{j,i} \quad (2r_T N_o^2) \quad (3862)$$

$$\tau^7_{\gamma,\delta,w} = \sum_{i \in O} {}^2D^4_{i,w} Y^{4,*}_{i,\delta} \tau^6_{\gamma,i} \quad (3r_D r_T^2 N_o) \quad (3875)$$

$$\tau^7_{\gamma,\delta,w} = \sum_{i \in O} {}^2D^4_{i,w} Y^{4,*}_{i,\delta} \tau^6_{\gamma,i} \quad (3r_D r_T^2 N_o) \quad (3863)$$

$$\tau^8_{\gamma,\delta,w} = \sum_{\epsilon \in A} Z^*_{\delta,\epsilon} \tau^1_{\gamma,\epsilon,w} \tau^7_{\gamma,\epsilon,w} \quad (3r_D r_T^3) \quad (3876)$$

$$\tau^8_{\gamma,\delta,w} = \sum_{\epsilon \in A} Z^*_{\delta,\epsilon} \tau^1_{\gamma,\epsilon,w} \tau^7_{\gamma,\epsilon,w} \quad (3r_D r_T^3) \quad (3864)$$

$$\tau^9_{\gamma,\delta,w} = \sum_{\epsilon \in A} Z_{\epsilon,\gamma} \tau^8_{\epsilon,\delta,w} \quad (2r_D r_T^3) \quad (3877)$$

$$\tau^9_{\gamma,\delta,w} = \sum_{\epsilon \in A} Z_{\gamma,\epsilon} \tau^8_{\epsilon,\delta,w} \quad (2r_D r_T^3) \quad (3865)$$

$${}^2R^2_{i,\gamma} \leftarrow \sum_{\delta \in A} \sum_{w \in D} \frac{1}{2} {}^2D^2_{i,w} Y^4_{i,\delta} \tau^0_{\delta,\gamma,w} \tau^9_{\delta,\gamma,w} \quad (4r_D r_T^2 N_o) \quad (3878)$$

$${}^2R^2_{i,\gamma} \leftarrow \sum_{\delta \in A} \sum_{w \in D} \frac{1}{2} {}^2D^2_{i,w} Y^2_{i,\delta} \tau^0_{\delta,\gamma,w} \tau^9_{\delta,\gamma,w} \quad (4r_D r_T^2 N_o) \quad (3866)$$

Raw expression

$${}^2R^2_{i,\epsilon} \leftarrow - \sum_{\gamma \in A} \sum_{j \in O} \sum_{k \in O} \sum_{a \in V} \sum_{b \in V} \sum_{c \in V} \sum_{d \in V} \frac{1}{2} {}^1T_{c,k} Y^{1,*}_{a,\epsilon} Z^*_{\epsilon,\gamma} Y^{3,*}_{b,\gamma} Y^{4,*}_{j,\gamma} {}^2D^{a,i,b,j} {}^2T_{d,j,a,i} V_{b,c,k,d} \quad (3867)$$

Factorized expression

$$\tau^0_{\gamma,\delta,w} = \sum_{a \in V} {}^2D^1_{a,w} Y^3_{a,\gamma} Y^{1,*}_{a,\delta} \quad (3r_D r_T^2 N_v) \quad (3868)$$

$$\tau^1_{\gamma,\delta,w} = \sum_{a \in V} {}^2D^3_{a,w} Y^1_{a,\gamma} Y^{3,*}_{a,\delta} \quad (3r_D r_T^2 N_v) \quad (3869)$$

Raw expression

$${}^2R^2_{i,\epsilon} \leftarrow \sum_{\gamma \in A} \sum_{j \in O} \sum_{k \in O} \sum_{l \in O} \sum_{a \in V} \sum_{b \in V} \sum_{c \in V} \frac{1}{2} {}^1T_{a,k} Y^{1,*}_{a,\epsilon} Z^*_{\epsilon,\gamma} Y^{3,*}_{b,\gamma} Y^{4,*}_{j,\gamma} {}^2D^{a,i,b,j} {}^2T_{b,j,c,l} V_{l,i,k,c} \quad (3879)$$

Factorized expression

$$\tau^0_{\gamma,\alpha,w} = \sum_{a \in V} {}^2D^1_{a,w} W^1_{a,\alpha} Y^{1,*}_{a,\gamma} \quad (3r_D r_T r_V N_v) \quad (3880)$$

$$\tau^1_{\gamma,\alpha} = \sum_{a \in V} W^4_{a,\alpha} Y^3_{a,\gamma} \quad (2r_T r_V N_v) \quad (3881)$$

$$\tau^2_{\gamma,\alpha} = \sum_{i \in O} W^3_{i,\alpha} Y^4_{i,\gamma} \quad (2r_T r_V N_o) \quad (3882)$$

$$\tau^3_{\gamma,\alpha} = \sum_{\beta \in B} X_{\alpha,\beta} \tau^1_{\gamma,\beta} \tau^2_{\gamma,\beta} \quad (3r_T r_V^2) \quad (3883)$$

$$\tau^4_{\gamma,\alpha} = \sum_{\delta \in A} Z_{\gamma,\delta} \tau^3_{\delta,\alpha} \quad (2r_T^2 r_V) \quad (3884)$$

$$\tau^5_{\gamma,\delta,w} = \sum_{a \in V} {}^2D^3_{a,w} Y^1_{a,\gamma} Y^{3,*}_{a,\delta} \quad (3r_D r_T^2 N_v) \quad (3885)$$

$$\tau^6_{\gamma,\delta,w} = \sum_{i \in O} {}^2D^4_{i,w} Y^2_{i,\gamma} Y^{4,*}_{i,\delta} \quad (3r_D r_T^2 N_o) \quad (3886)$$

$$\tau^7_{\gamma,\delta,w} = \sum_{\epsilon \in A} Z^*_{\delta,\epsilon} \tau^5_{\gamma,\epsilon,w} \tau^6_{\gamma,\epsilon,w} \quad (3r_D r_T^3) \quad (3887)$$

$$\tau^8_{\gamma,\alpha,w} = \sum_{\delta \in A} \tau^4_{\delta,\alpha} \tau^7_{\delta,\gamma,w} \quad (2r_D r_T^2 r_V) \quad (3888)$$

$$\tau^9_{\alpha,i} = \sum_{a \in V} {}^1T_{a,i} W^2_{a,\alpha} \quad (2r_V N_o N_v) \quad (3889)$$

$$\tau^{10}_{\gamma,w,i} = \sum_{\alpha \in B} \tau^9_{\alpha,i} \tau^0_{\gamma,\alpha,w} \tau^8_{\gamma,\alpha,w} \quad (3r_D r_T r_V N_o) \quad (3890)$$

$${}^2R^2_{i,\gamma} \leftarrow \sum_{w \in D} {}^2D^2_{i,w} \tau^{10}_{\gamma,w,i} \quad (2r_D r_T N_o) \quad (3891)$$

Raw expression

$${}^2R^2_{i,\epsilon} \leftarrow \sum_{\gamma \in A} \sum_{j \in O} \sum_{k \in O} \sum_{l \in O} \sum_{a \in V} \sum_{b \in V} \sum_{c \in V} \frac{1}{2} {}^1T_{a,k} Y^{1,*}_{a,\epsilon} Z^*_{\epsilon,\gamma} Y^{3,*}_{b,\gamma} Y^{4,*}_{j,\gamma} {}^2D^{a,i,b,j} {}^2T_{b,l,c,i} V_{k,c,l,j} \quad (3892)$$

Factorized expression

$$\tau^0_{\gamma,\alpha,w} = \sum_{a \in V} {}^2D^1_{a,w} W^1_{a,\alpha} Y^{1,*}_{a,\gamma} \quad (3r_D r_T r_V N_v) \quad (3893)$$

$$\tau^1_{\gamma,\delta,w} = \sum_{a \in V} {}^2D^3_{a,w} Y^3_{a,\gamma} Y^{3,*}_{a,\delta} \quad (3r_D r_T^2 N_v) \quad (3894)$$

$$\tau^2_{\gamma,\delta,w} = \sum_{i \in O} {}^2D^4_{i,w} Y^4_{i,\gamma} Y^{4,*}_{i,\delta} \quad (3r_D r_T^2 N_o) \quad (3895)$$

$$\tau^3_{\gamma,\delta,w} = \sum_{\epsilon \in A} Z^*_{\delta,\epsilon} \tau^1_{\gamma,\epsilon,w} \tau^2_{\gamma,\epsilon,w} \quad (3r_D r_T^3) \quad (3896)$$

$$\tau^4_{\gamma,\alpha} = \sum_{a \in V} W^4_{a,\alpha} Y^1_{a,\gamma} \quad (2r_T r_V N_v) \quad (3897)$$

$$\tau^5_{\gamma,\alpha} = \sum_{i \in O} W^3_{i,\alpha} Y^2_{i,\gamma} \quad (2r_T r_V N_o) \quad (3898)$$

$$\tau^6_{\gamma,\alpha} = \sum_{\beta \in B} X_{\alpha,\beta} \tau^4_{\gamma,\beta} \tau^5_{\gamma,\beta} \quad (3r_T r_V^2) \quad (3899)$$

$$\tau^7_{\gamma,\alpha} = \sum_{\delta \in A} Z_{\delta,\gamma} \tau^6_{\delta,\alpha} \quad (2r_T^2 r_V) \quad (3900)$$

$$\tau^8_{\gamma,\alpha,w} = \sum_{\delta \in A} \tau^7_{\delta,\alpha} \tau^3_{\delta,\gamma,w} \quad (2r_D r_T^2 r_V) \quad (3901)$$

$$\tau^9_{\alpha,i} = \sum_{a \in V} {}^1T_{a,i} W^2_{a,\alpha} \quad (2r_V N_o N_v) \quad (3902)$$

$$\tau^{10}_{\gamma,w,i} = \sum_{\alpha \in B} \tau^9_{\alpha,i} \tau^0_{\gamma,\alpha,w} \tau^8_{\gamma,\alpha,w} \quad (3r_D r_T r_V N_o) \quad (3903)$$

$${}^2R^2_{i,\gamma} \leftarrow \sum_{w \in D} {}^2D^2_{i,w} \tau^{10}_{\gamma,w,i} \quad (2r_D r_T N_o) \quad (3904)$$

Raw expression

$${}^2R^2_{i,\epsilon} \leftarrow \sum_{\gamma \in A} \sum_{j \in O} \sum_{k \in O} \sum_{l \in O} \sum_{a \in V} \sum_{b \in V} \sum_{c \in V} \frac{1}{2} {}^1T_{a,k} Y^{1,*}_{a,\epsilon} Z^*_{\epsilon,\gamma} Y^{3,*}_{b,\gamma} Y^{4,*}_{j,\gamma} {}^2D^{a,i,b,j} {}^2T_{b,l,c,j} V_{k,i,l,c} \quad (3905)$$

Factorized expression

$$\tau^0_{\gamma,\delta,w} = \sum_{a \in V} {}^2D^1_{a,w} Y^1_{a,\gamma} Y^{1,*}_{a,\delta} \quad (3r_D r_T^2 N_v) \quad (3906)$$

$$\tau^1_{\alpha,i} = \sum_{a \in V} {}^1T_{a,i} W^2_{a,\alpha} \quad (2r_V N_o N_v) \quad (3907)$$

$$\tau^2_{\gamma,\alpha,w} = \sum_{i \in O} {}^2D^4_{i,w} Y^{4,*}_{i,\gamma} \tau^1_{\alpha,i} \quad (3r_D r_T r_V N_o) \quad (3908)$$

$$\tau^3_{\gamma,\alpha,w} = \sum_{a \in V} {}^2D^3_{a,w} W^1_{a,\alpha} Y^{3,*}_{a,\gamma} \quad (3r_D r_T r_V N_v) \quad (3909)$$

$$\tau^4_{\gamma,\alpha} = \sum_{a \in V} W^4_{a,\alpha} Y^3_{a,\gamma} \quad (2r_T r_V N_v) \quad (3910)$$

$$\tau^5_{\gamma,\alpha} = \sum_{i \in O} W^3_{i,\alpha} Y^4_{i,\gamma} \quad (2r_T r_V N_o) \quad (3911)$$

$$\tau^6_{\gamma,\alpha} = \sum_{\beta \in B} X_{\alpha,\beta} \tau^4_{\gamma,\beta} \tau^5_{\gamma,\beta} \quad (3r_T r_V^2) \quad (3912)$$

$$\tau^7_{\gamma,\alpha} = \sum_{\delta \in A} Z_{\delta,\gamma} \tau^6_{\delta,\alpha} \quad (2r_T^2 r_V) \quad (3913)$$

$$\tau^8_{\gamma,\delta,w} = \sum_{\alpha \in B} \tau^7_{\gamma,\alpha} \tau^2_{\delta,\alpha,w} \tau^3_{\delta,\alpha,w} \quad (3r_D r_T^2 r_V) \quad (3914)$$

$$\tau^9_{\gamma,\delta,w} = \sum_{\epsilon \in A} Z^*_{\delta,\epsilon} \tau^8_{\gamma,\epsilon,w} \quad (2r_D r_T^3) \quad (3915)$$

$${}^2R^2_{i,\gamma} \leftarrow \sum_{\delta \in A} \sum_{w \in D} {}^2D^2_{i,w} Y^2_{i,\delta} \tau^0_{\delta,\gamma,w} \tau^9_{\delta,\gamma,w} \quad (4r_D r_T^2 N_o) \quad (3916)$$

Raw expression

$${}^2R^2_{i,\epsilon} \leftarrow \sum_{\gamma \in A} \sum_{j \in O} \sum_{k \in O} \sum_{l \in O} \sum_{a \in V} \sum_{b \in V} \sum_{c \in V} \frac{1}{2} {}^1T_{a,k} Y^{1,*}_{a,\epsilon} Z^*_{\epsilon,\gamma} Y^{3,*}_{b,\gamma} Y^{4,*}_{j,\gamma} {}^2D^{a,i,b,j} {}^2T_{c,i,b,l} V_{k,c,l,j} \quad (3917)$$

Factorized expression

$$\tau^0_{\gamma,\delta,w} = \sum_{a \in V} {}^2D^1_{a,w} Y^3_{a,\gamma} Y^{1,*}_{a,\delta} \quad (3r_D r_T^2 N_v) \quad (3918)$$

$$\tau^1_{\alpha,i} = \sum_{a \in V} {}^1T_{a,i} W^2_{a,\alpha} \quad (2r_V N_o N_v) \quad (3919)$$

$$\tau^2_{\gamma,\alpha,w} = \sum_{i \in O} {}^2D^4_{i,w} Y^{4,*}_{i,\gamma} \tau^1_{\alpha,i} \quad (3r_D r_T r_V N_o) \quad (3920)$$

$$\tau^3_{\gamma,\alpha,w} = \sum_{a \in V} {}^2D^3_{a,w} W^1_{a,\alpha} Y^{3,*}_{a,\gamma} \quad (3r_D r_T r_V N_v) \quad (3921)$$

$$\tau^4_{\gamma,\alpha} = \sum_{a \in V} W^4_{a,\alpha} Y^1_{a,\gamma} \quad (2r_T r_V N_v) \quad (3922)$$

$$\tau^5_{\gamma,\alpha} = \sum_{i \in O} W^3_{i,\alpha} Y^2_{i,\gamma} \quad (2r_T r_V N_o) \quad (3923)$$

$$\tau^6_{\gamma,\alpha} = \sum_{\beta \in B} X_{\alpha,\beta} \tau^4_{\gamma,\beta} \tau^5_{\gamma,\beta} \quad (3r_T r_V^2) \quad (3924)$$

$$\tau^7_{\gamma,\alpha} = \sum_{\delta \in A} Z_{\delta,\gamma} \tau^6_{\delta,\alpha} \quad (2r_T^2 r_V) \quad (3925)$$

$$\tau^8_{\gamma,\delta,w} = \sum_{\alpha \in B} \tau^7_{\gamma,\alpha} \tau^2_{\delta,\alpha,w} \tau^3_{\delta,\alpha,w} \quad (3r_D r_T^2 r_V) \quad (3926)$$

$$\tau^9_{\gamma,\delta,w} = \sum_{\epsilon \in A} Z^*_{\delta,\epsilon} \tau^8_{\gamma,\epsilon,w} \quad (2r_D r_T^3) \quad (3927)$$

$${}^2R^2_{i,\gamma} \leftarrow \sum_{\delta \in A} \sum_{w \in D} {}^2D^2_{i,w} Y^4_{i,\delta} \tau^0_{\delta,\gamma,w} \tau^9_{\delta,\gamma,w} \quad (4r_D r_T^2 N_o) \quad (3928)$$

Raw expression

$${}^2R^2_{i,\epsilon} \leftarrow \sum_{\gamma \in A} \sum_{j \in O} \sum_{k \in O} \sum_{l \in O} \sum_{a \in V} \sum_{b \in V} \sum_{c \in V} \frac{1}{2} {}^1T_{a,k} Y^{1,*}_{a,\epsilon} Z^*_{\epsilon,\gamma} Y^{3,*}_{b,\gamma} Y^{4,*}_{j,\gamma} {}^2D^{a,i,b,j} {}^2T_{c,j,b,l} V_{k,i,l,c} \quad (3929)$$

Factorized expression

$$\tau^0_{\gamma,\delta,w} = \sum_{a \in V} {}^2D^3_{a,w} Y^1_{a,\gamma} Y^{3,*}_{a,\delta} \quad (3r_D r_T^2 N_v) \quad (3930)$$

$$\tau^1_{\gamma,\delta,w} = \sum_{i \in O} {}^2D^4_{i,w} Y^2_{i,\gamma} Y^{4,*}_{i,\delta} \quad (3r_D r_T^2 N_o) \quad (3931)$$

$$\tau^2_{\gamma,\delta,w} = \sum_{\epsilon \in A} Z^*_{\delta,\epsilon} \tau^0_{\gamma,\epsilon,w} \tau^1_{\gamma,\epsilon,w} \quad (3r_D r_T^3) \quad (3932)$$

$$\tau^3_{\gamma,\delta,w} = \sum_{\epsilon \in A} Z_{\epsilon,\gamma} \tau^2_{\epsilon,\delta,w} \quad (2r_D r_T^3) \quad (3933)$$

$$\tau^4_{\alpha,i} = \sum_{a \in V} {}^1T_{a,i} W^4_{a,\alpha} \quad (2r_V N_o N_v) \quad (3934)$$

$$\tau^5_\alpha = \sum_{i \in O} W^3_{i,\alpha} \tau^4_{\alpha,i} \quad (2r_V N_o) \quad (3935)$$

$$\tau^6_\alpha = \sum_{\beta \in B} \tau^5_\beta X_{\alpha,\beta} \quad (2r_V^2) \quad (3948)$$

$$\tau^6_\alpha = \sum_{\beta \in B} \tau^5_\beta X_{\alpha,\beta} \quad (2r_V^2) \quad (3936)$$

$$\tau^7_{a,b} = \sum_{\alpha \in B} \tau^6_\alpha W^1_{a,\alpha} W^2_{b,\alpha} \quad (3r_V N_v^2) \quad (3949)$$

$$\tau^7_{a,b} = \sum_{\alpha \in B} \tau^6_\alpha W^1_{a,\alpha} W^2_{b,\alpha} \quad (3r_V N_v^2) \quad (3937)$$

$$\tau^8_{\gamma,a} = \sum_{b \in V} Y^1_{b,\gamma} \tau^7_{a,b} \quad (2r_T N_v^2) \quad (3950)$$

$$\tau^8_{\gamma,a} = \sum_{b \in V} Y^3_{b,\gamma} \tau^7_{a,b} \quad (2r_T N_v^2) \quad (3938)$$

$$\tau^9_{\gamma,\delta,w} = \sum_{a \in V} {}^2D^1_{a,w} Y^{1,*}_{a,\delta} \tau^8_{\gamma,a} \quad (3r_D r_T^2 N_v) \quad (3951)$$

$$\tau^9_{\gamma,\delta,w} = \sum_{a \in V} {}^2D^1_{a,w} Y^{1,*}_{a,\delta} \tau^8_{\gamma,a} \quad (3r_D r_T^2 N_v) \quad (3939)$$

$${}^2R^2_{i,\gamma} \leftarrow \sum_{\delta \in A} \sum_{w \in D} {}^2D^2_{i,w} Y^2_{i,\delta} \tau^3_{\delta,\gamma,w} \tau^9_{\delta,\gamma,w} \quad (4r_D r_T^2 N_o) \quad (3952)$$

$${}^2R^2_{i,\gamma} \leftarrow \sum_{\delta \in A} \sum_{w \in D} {}^2D^2_{i,w} Y^4_{i,\delta} \tau^3_{\delta,\gamma,w} \tau^9_{\delta,\gamma,w} \quad (4r_D r_T^2 N_o) \quad (3940)$$

Raw expression

$${}^2R^2_{i,\epsilon} \leftarrow \sum_{\gamma \in A} \sum_{j \in O} \sum_{k \in O} \sum_{l \in O} \sum_{a \in V} \sum_{b \in V} \sum_{c \in V} \frac{1}{2} {}^1T_{b,k} Y^{1,*}_{a,\epsilon} Z^*_{\epsilon,\gamma} Y^{3,*}_{b,\gamma} Y^{4,*}_{j,\gamma} {}^2D^{a,i,b,j} {}^2T_{a,i,c,l} V_{k,c,l,j} \quad (3953)$$

Raw expression

$${}^2R^2_{i,\epsilon} \leftarrow \sum_{\gamma \in A} \sum_{j \in O} \sum_{k \in O} \sum_{l \in O} \sum_{a \in V} \sum_{b \in V} \sum_{c \in V} \frac{1}{2} {}^1T_{a,k} Y^{1,*}_{a,\epsilon} Z^*_{\epsilon,\gamma} Y^{3,*}_{b,\gamma} Y^{4,*}_{j,\gamma} {}^2D^{a,i,b,j} {}^2T_{c,l,b,j} V_{l,i,k,c} \quad (3941)$$

Factorized expression

$$\tau^0_{\gamma,\delta,w} = \sum_{a \in V} {}^2D^1_{a,w} Y^1_{a,\gamma} Y^{1,*}_{a,\delta} \quad (3r_D r_T^2 N_v) \quad (3954)$$

Factorized expression

$$\tau^0_{\gamma,\delta,w} = \sum_{a \in V} {}^2D^3_{a,w} Y^3_{a,\gamma} Y^{3,*}_{a,\delta} \quad (3r_D r_T^2 N_v) \quad (3942)$$

$$\tau^1_{\gamma,\delta,w} = \sum_{i \in O} {}^2D^4_{i,w} Y^4_{i,\gamma} Y^{4,*}_{i,\delta} \quad (3r_D r_T^2 N_o) \quad (3955)$$

$$\tau^1_{\gamma,\delta,w} = \sum_{i \in O} {}^2D^4_{i,w} Y^4_{i,\gamma} Y^{4,*}_{i,\delta} \quad (3r_D r_T^2 N_o) \quad (3943)$$

$$\tau^2_{\alpha,i} = \sum_{a \in V} {}^1T_{a,i} W^4_{a,\alpha} \quad (2r_V N_o N_v) \quad (3956)$$

$$\tau^2_{\gamma,\delta,w} = \sum_{\epsilon \in A} Z^*_{\delta,\epsilon} \tau^0_{\gamma,\epsilon,w} \tau^1_{\gamma,\epsilon,w} \quad (3r_D r_T^3) \quad (3944)$$

$$\tau^3_\alpha = \sum_{i \in O} W^3_{i,\alpha} \tau^2_{\alpha,i} \quad (2r_V N_o) \quad (3957)$$

$$\tau^3_{\gamma,\delta,w} = \sum_{\epsilon \in A} Z_{\gamma,\epsilon} \tau^2_{\epsilon,\delta,w} \quad (2r_D r_T^3) \quad (3945)$$

$$\tau^4_\alpha = \sum_{\beta \in B} \tau^3_\beta X_{\alpha,\beta} \quad (2r_V^2) \quad (3958)$$

$$\tau^4_{\alpha,i} = \sum_{a \in V} {}^1T_{a,i} W^4_{a,\alpha} \quad (2r_V N_o N_v) \quad (3946)$$

$$\tau^5_{a,b} = \sum_{\alpha \in B} \tau^4_\alpha W^1_{a,\alpha} W^2_{b,\alpha} \quad (3r_V N_v^2) \quad (3959)$$

$$\tau^5_\alpha = \sum_{i \in O} W^3_{i,\alpha} \tau^4_{\alpha,i} \quad (2r_V N_o) \quad (3947)$$

$$\tau^6_{\gamma,a} = \sum_{b \in V} Y^3_{b,\gamma} \tau^5_{a,b} \quad (2r_T N_v^2) \quad (3960)$$

$$\tau^7_{\gamma,\delta,w} = \sum_{a \in V} {}^2D^3_{a,w} Y^{3,*}_{a,\delta} \tau^6_{\gamma,a} \quad (3r_D r_T^2 N_v) \quad (3961)$$

$$\tau^8_{\gamma,\delta,w} = \sum_{\epsilon \in A} Z_{\epsilon,\gamma} \tau^7_{\epsilon,\delta,w} \quad (2r_D r_T^3) \quad (3974)$$

$$\tau^8_{\gamma,\delta,w} = \sum_{\epsilon \in A} Z^*_{\delta,\epsilon} \tau^1_{\gamma,\epsilon,w} \tau^7_{\gamma,\epsilon,w} \quad (3r_D r_T^3) \quad (3962)$$

$$\tau^9_{\gamma,\delta,w} = \sum_{a \in V} {}^2D^1_{a,w} Y^3_{a,\gamma} Y^{1,*}_{a,\delta} \quad (3r_D r_T^2 N_v) \quad (3975)$$

$$\tau^9_{\gamma,\delta,w} = \sum_{\epsilon \in A} Z_{\gamma,\epsilon} \tau^8_{\epsilon,\delta,w} \quad (2r_D r_T^3) \quad (3963)$$

$${}^2R^2_{i,\gamma} \leftarrow \sum_{\delta \in A} \sum_{w \in D} {}^2D^2_{i,w} Y^4_{i,\delta} \tau^8_{\delta,\gamma,w} \tau^9_{\delta,\gamma,w} \quad (4r_D r_T^2 N_o) \quad (3976)$$

$${}^2R^2_{i,\gamma} \leftarrow \sum_{\delta \in A} \sum_{w \in D} {}^2D^2_{i,w} Y^2_{i,\delta} \tau^0_{\delta,\gamma,w} \tau^9_{\delta,\gamma,w} \quad (4r_D r_T^2 N_o) \quad (3964)$$

Raw expression

$${}^2R^2_{i,\epsilon} \leftarrow \sum_{\gamma \in A} \sum_{j \in O} \sum_{k \in O} \sum_{l \in O} \sum_{a \in V} \sum_{b \in V} \sum_{c \in V} \frac{1}{2} {}^1T_{b,k} Y^{1,*}_{a,\epsilon} Z^*_{\epsilon,\gamma} Y^{3,*}_{b,\gamma} Y^{4,*}_{j,\gamma} {}^2D^{a,i,b,j} {}^2T_{a,l,c,i} V_{l,c,k,j} \quad (3965)$$

Factorized expression

$$\tau^0_{\gamma,\delta,w} = \sum_{i \in O} {}^2D^4_{i,w} Y^2_{i,\gamma} Y^{4,*}_{i,\delta} \quad (3r_D r_T^2 N_o) \quad (3966)$$

$$\tau^1_{\alpha,i} = \sum_{a \in V} {}^1T_{a,i} W^4_{a,\alpha} \quad (2r_V N_o N_v) \quad (3967)$$

$$\tau^2_{\alpha} = \sum_{i \in O} W^3_{i,\alpha} \tau^1_{\alpha,i} \quad (2r_V N_o) \quad (3968)$$

$$\tau^3_{\alpha} = \sum_{\beta \in B} \tau^2_{\beta} X_{\alpha,\beta} \quad (2r_V^2) \quad (3969)$$

$$\tau^4_{a,b} = \sum_{\alpha \in B} \tau^3_{\alpha} W^1_{a,\alpha} W^2_{b,\alpha} \quad (3r_V N_v^2) \quad (3970)$$

$$\tau^5_{\gamma,a} = \sum_{b \in V} Y^1_{b,\gamma} \tau^4_{a,b} \quad (2r_T N_v^2) \quad (3971)$$

$$\tau^6_{\gamma,\delta,w} = \sum_{a \in V} {}^2D^3_{a,w} Y^{3,*}_{a,\delta} \tau^5_{\gamma,a} \quad (3r_D r_T^2 N_v) \quad (3972)$$

$$\tau^7_{\gamma,\delta,w} = \sum_{\epsilon \in A} Z^*_{\delta,\epsilon} \tau^0_{\gamma,\epsilon,w} \tau^6_{\gamma,\epsilon,w} \quad (3r_D r_T^3) \quad (3973)$$

Raw expression

$${}^2R^2_{i,\epsilon} \leftarrow \sum_{\gamma \in A} \sum_{j \in O} \sum_{k \in O} \sum_{l \in O} \sum_{a \in V} \sum_{b \in V} \sum_{c \in V} \frac{1}{2} {}^1T_{b,k} Y^{1,*}_{a,\epsilon} Z^*_{\epsilon,\gamma} Y^{3,*}_{b,\gamma} Y^{4,*}_{j,\gamma} {}^2D^{a,i,b,j} {}^2T_{a,l,c,j} V_{l,i,k,c} \quad (3977)$$

Factorized expression

$$\tau^0_{\gamma,\alpha,w} = \sum_{a \in V} {}^2D^3_{a,w} W^1_{a,\alpha} Y^{3,*}_{a,\gamma} \quad (3r_D r_T r_V N_v) \quad (3978)$$

$$\tau^1_{\gamma,\alpha} = \sum_{a \in V} W^2_{a,\alpha} Y^1_{a,\gamma} \quad (2r_T r_V N_v) \quad (3979)$$

$$\tau^2_{\gamma,\alpha,i} = \sum_{\delta \in A} Y^2_{i,\delta} Z_{\delta,\gamma} \tau^1_{\delta,\alpha} \quad (3r_T^2 r_V N_o) \quad (3980)$$

$$\tau^3_{\gamma,\delta,\alpha,w} = \sum_{i \in O} {}^2D^4_{i,w} Y^{4,*}_{i,\delta} \tau^0_{\delta,\alpha,w} \tau^2_{\gamma,\alpha,i} \quad (4r_D r_T^2 r_V N_o) \quad (3981)$$

$$\tau^4_{\gamma,\alpha} = \sum_{a \in V} W^4_{a,\alpha} Y^3_{a,\gamma} \quad (2r_T r_V N_v) \quad (3982)$$

$$\tau^5_{\gamma,\alpha,i} = \sum_{\beta \in B} X_{\alpha,\beta} W^3_{i,\beta} \tau^4_{\gamma,\beta} \quad (3r_T r_V^2 N_o) \quad (3983)$$

$$\tau^6_{\gamma,\delta,w,i} = \sum_{\alpha \in B} \tau^5_{\gamma,\alpha,i} \tau^3_{\gamma,\delta,\alpha,w} \quad (2r_D r_T^2 r_V N_o) \quad (3984)$$

$$\tau^7_{\gamma,w,i,j} = \sum_{\delta \in A} {}^2D^2_{i,w} Y^4_{i,\delta} \tau^6_{\delta,\gamma,w,j} \quad (3r_D r_T^2 N_o^2) \quad (3985)$$

$$\tau_{\gamma,w,i}^8 = \sum_{a \in V} {}^2D_{a,w}^1 T_{a,i} Y_{a,\gamma}^{1,*} \quad (3r_D r_T N_o N_v) \quad (3986)$$

$$\tau_{\gamma,w,i}^8 = \sum_{a \in V} {}^2D_{a,w}^1 T_{a,i} Y_{a,\gamma}^{1,*} \quad (3r_D r_T N_o N_v) \quad (3998)$$

$$\tau_{\gamma,\delta,i}^9 = \sum_{w \in D} \sum_{j \in O} \tau_{\gamma,w,j}^8 \tau_{\delta,w,i,j}^7 \quad (2r_D r_T^2 N_o^2) \quad (3987)$$

$$\tau_{\gamma,\delta,i}^9 = \sum_{w \in D} \sum_{j \in O} \tau_{\gamma,w,j}^8 \tau_{\delta,w,i,j}^7 \quad (2r_D r_T^2 N_o^2) \quad (3999)$$

$${}^2R_{i,\gamma}^2 \leftarrow - \sum_{\delta \in A} \frac{1}{2} Z_{\gamma,\delta}^* \tau_{\gamma,\delta,i}^9 \quad (2r_T^2 N_o) \quad (3988)$$

$${}^2R_{i,\gamma}^2 \leftarrow - \sum_{\delta \in A} \frac{1}{2} Z_{\gamma,\delta}^* \tau_{\gamma,\delta,i}^9 \quad (2r_T^2 N_o) \quad (4000)$$

Raw expression

$${}^2R_{i,\epsilon}^2 \leftarrow \sum_{\gamma \in A} \sum_{j \in O} \sum_{k \in O} \sum_{l \in O} \sum_{a \in V} \sum_{b \in V} \sum_{c \in V} \frac{1}{2} {}^1T_{b,k} Y_{a,\epsilon}^{1,*} Z_{\epsilon,\gamma}^* Y_{b,\gamma}^{3,*} Y_{j,\gamma}^{4,*} {}^2D_{a,i,b,j} {}^2T_{c,i,a,l} V_{l,c,k,j} \quad (3989)$$

Raw expression

$${}^2R_{i,\epsilon}^2 \leftarrow \sum_{\gamma \in A} \sum_{j \in O} \sum_{k \in O} \sum_{l \in O} \sum_{a \in V} \sum_{b \in V} \sum_{c \in V} \frac{1}{2} {}^1T_{b,k} Y_{a,\epsilon}^{1,*} Z_{\epsilon,\gamma}^* Y_{b,\gamma}^{3,*} Y_{j,\gamma}^{4,*} {}^2D_{a,i,b,j} {}^2T_{c,j,a,l} V_{l,i,k,c} \quad (4001)$$

Factorized expression

$$\tau_{\gamma,\alpha,w}^0 = \sum_{a \in V} {}^2D_{a,w}^3 W_{a,\alpha}^1 Y_{a,\gamma}^{3,*} \quad (3r_D r_T r_V N_v) \quad (3990)$$

$$\tau_{\gamma,\alpha}^0 = \sum_{a \in V} W_{a,\alpha}^2 Y_{a,\gamma}^1 \quad (2r_T r_V N_v) \quad (4002)$$

$$\tau_{\gamma,\alpha}^1 = \sum_{a \in V} W_{a,\alpha}^2 Y_{a,\gamma}^3 \quad (2r_T r_V N_v) \quad (3991)$$

$$\tau_{\gamma,\alpha,i}^1 = \sum_{\delta \in A} Y_{i,\delta}^2 Z_{\delta,\gamma} \tau_{\delta,\alpha}^0 \quad (3r_T^2 r_V N_o) \quad (4003)$$

$$\tau_{\gamma,\alpha,i}^2 = \sum_{\delta \in A} Z_{\gamma,\delta} Y_{i,\delta}^4 \tau_{\delta,\alpha}^1 \quad (3r_T^2 r_V N_o) \quad (3992)$$

$$\tau_{\gamma,w,i}^2 = \sum_{a \in V} {}^2D_{a,w}^3 T_{a,i} Y_{a,\gamma}^{3,*} \quad (3r_D r_T N_o N_v) \quad (4004)$$

$$\tau_{\gamma,\delta,\alpha,w}^3 = \sum_{i \in O} {}^2D_{i,w}^4 Y_{i,\delta}^{4,*} \tau_{\delta,\alpha,w}^0 \tau_{\gamma,\alpha,i}^2 \quad (4r_D r_T^2 r_V N_o) \quad (3993)$$

$$\tau_{\gamma,w,i,j}^3 = \sum_{\delta \in A} Z_{\gamma,\delta}^* Y_{j,\delta}^{4,*} \tau_{\delta,w,i}^2 \quad (3r_D r_T^2 N_o^2) \quad (4005)$$

$$\tau_{\gamma,\alpha}^4 = \sum_{a \in V} W_{a,\alpha}^4 Y_{a,\gamma}^1 \quad (2r_T r_V N_v) \quad (3994)$$

$$\tau_{\gamma,\delta,w,i}^4 = \sum_{j \in O} {}^2D_{j,w}^4 Y_{j,\gamma}^4 \tau_{\delta,w,i,j}^3 \quad (3r_D r_T^2 N_o^2) \quad (4006)$$

$$\tau_{\gamma,\alpha,i}^5 = \sum_{\beta \in B} X_{\alpha,\beta} W_{i,\beta}^3 \tau_{\gamma,\beta}^4 \quad (3r_T r_V^2 N_o) \quad (3995)$$

$$\tau_{\gamma,\alpha}^5 = \sum_{a \in V} W_{a,\alpha}^4 Y_{a,\gamma}^3 \quad (2r_T r_V N_v) \quad (4007)$$

$$\tau_{\gamma,\delta,w,i}^6 = \sum_{\alpha \in B} \tau_{\gamma,\alpha,i}^5 \tau_{\gamma,\delta,\alpha,w}^3 \quad (2r_D r_T^2 r_V N_o) \quad (3996)$$

$$\tau_{\gamma,\alpha,i}^6 = \sum_{\beta \in B} X_{\alpha,\beta} W_{i,\beta}^3 \tau_{\gamma,\beta}^5 \quad (3r_T r_V^2 N_o) \quad (4008)$$

$$\tau_{\gamma,w,i,j}^7 = \sum_{\delta \in A} {}^2D_{i,w}^2 Y_{i,\delta}^2 \tau_{\delta,\gamma,w,j}^6 \quad (3r_D r_T^2 N_o^2) \quad (3997)$$

$$\tau_{\gamma,\delta,\alpha,w}^7 = \sum_{i \in O} \tau_{\gamma,\alpha,i}^6 \tau_{\gamma,\delta,w,i}^4 \quad (2r_D r_T^2 r_V N_o) \quad (4009)$$

$$\tau^8_{\gamma,\alpha,w,i} = \sum_{\delta \in A} \tau^1_{\delta,\alpha,i} \tau^7_{\delta,\gamma,\alpha,w} \quad (2r_D r_T^2 r_V N_o) \quad (4010)$$

$$\tau^7_{\gamma,\delta,\alpha,w} = \sum_{i \in O} \tau^6_{\gamma,\alpha,i} \tau^4_{\gamma,\delta,w,i} \quad (2r_D r_T^2 r_V N_o) \quad (4022)$$

$$\tau^9_{\gamma,\alpha,w} = \sum_{a \in V} {}^2D^1_{a,w} W^1_{a,\alpha} Y^{1,*}_{a,\gamma} \quad (3r_D r_T r_V N_v) \quad (4011)$$

$$\tau^8_{\gamma,\alpha,w,i} = \sum_{\delta \in A} \tau^1_{\delta,\alpha,i} \tau^7_{\delta,\gamma,\alpha,w} \quad (2r_D r_T^2 r_V N_o) \quad (4023)$$

$$\tau^{10}_{\gamma,w,i} = \sum_{\alpha \in B} \tau^9_{\gamma,\alpha,w} \tau^8_{\gamma,\alpha,w,i} \quad (2r_D r_T r_V N_o) \quad (4012)$$

$$\tau^9_{\gamma,\alpha,w} = \sum_{a \in V} {}^2D^1_{a,w} W^1_{a,\alpha} Y^{1,*}_{a,\gamma} \quad (3r_D r_T r_V N_v) \quad (4024)$$

$${}^2R^2_{i,\gamma} \leftarrow - \sum_{w \in D} \frac{1}{2} {}^2D^2_{i,w} \tau^{10}_{\gamma,w,i} \quad (2r_D r_T N_o) \quad (4013)$$

$$\tau^{10}_{\gamma,w,i} = \sum_{\alpha \in B} \tau^9_{\gamma,\alpha,w} \tau^8_{\gamma,\alpha,w,i} \quad (2r_D r_T r_V N_o) \quad (4025)$$

Raw expression

$${}^2R^2_{i,\gamma} \leftarrow - \sum_{w \in D} \frac{1}{2} {}^2D^2_{i,w} \tau^{10}_{\gamma,w,i} \quad (2r_D r_T N_o) \quad (4026)$$

$${}^2R^2_{i,\epsilon} \leftarrow \sum_{\gamma \in A} \sum_{j \in O} \sum_{k \in O} \sum_{l \in O} \sum_{a \in V} \sum_{b \in V} \sum_{c \in V} \frac{1}{2} {}^1T_{b,k} Y^{1,*}_{a,\epsilon} Z^*_{\epsilon,\gamma} Y^{3,*}_{b,\gamma} Y^{4,*}_{j,\gamma} {}^2D^{a,i,b,j} {}^2T_{c,l,a,i} V_{k,c,l,j} \quad (4014)$$

Raw expression

$${}^2R^2_{i,\epsilon} \leftarrow \sum_{\gamma \in A} \sum_{j \in O} \sum_{k \in O} \sum_{l \in O} \sum_{a \in V} \sum_{b \in V} \sum_{c \in V} \frac{1}{2} {}^1T_{c,i} Y^{1,*}_{a,\epsilon} Z^*_{\epsilon,\gamma} Y^{3,*}_{b,\gamma} Y^{4,*}_{j,\gamma} {}^2D^{a,i,b,j} {}^2T_{a,k,b,l} V_{k,c,l,j} \quad (4027)$$

Factorized expression

Factorized expression

$$\tau^0_{\gamma,\alpha} = \sum_{a \in V} W^2_{a,\alpha} Y^3_{a,\gamma} \quad (2r_T r_V N_v) \quad (4015)$$

$$\tau^0_{\gamma,\alpha,w} = \sum_{a \in V} {}^2D^1_{a,w} W^1_{a,\alpha} Y^{1,*}_{a,\gamma} \quad (3r_D r_T r_V N_v) \quad (4028)$$

$$\tau^1_{\gamma,\alpha,i} = \sum_{\delta \in A} Z_{\gamma,\delta} Y^4_{i,\delta} \tau^0_{\delta,\alpha} \quad (3r_T^2 r_V N_o) \quad (4016)$$

$$\tau^1_{\gamma,\delta,w} = \sum_{a \in V} {}^2D^3_{a,w} Y^1_{a,\gamma} Y^{3,*}_{a,\delta} \quad (3r_D r_T^2 N_v) \quad (4029)$$

$$\tau^2_{\gamma,w,i} = \sum_{a \in V} {}^2D^3_{a,w} {}^1T_{a,i} Y^{3,*}_{a,\gamma} \quad (3r_D r_T N_o N_v) \quad (4017)$$

$$\tau^2_{\gamma,\alpha} = \sum_{i \in O} W^3_{i,\alpha} Y^2_{i,\gamma} \quad (2r_T r_V N_o) \quad (4030)$$

$$\tau^3_{\gamma,w,i,j} = \sum_{\delta \in A} Z^*_{\gamma,\delta} Y^{4,*}_{j,\delta} \tau^2_{\delta,w,i} \quad (3r_D r_T^2 N_o^2) \quad (4018)$$

$$\tau^3_{\gamma,\alpha} = \sum_{a \in V} W^4_{a,\alpha} Y^3_{a,\gamma} \quad (2r_T r_V N_v) \quad (4031)$$

$$\tau^4_{\gamma,\delta,w,i} = \sum_{j \in O} {}^2D^4_{j,w} Y^2_{j,\gamma} \tau^3_{\delta,w,i,j} \quad (3r_D r_T^2 N_o^2) \quad (4019)$$

$$\tau^4_{\gamma,\alpha,i} = \sum_{\delta \in A} Z_{\gamma,\delta} Y^4_{i,\delta} \tau^3_{\delta,\alpha} \quad (3r_T^2 r_V N_o) \quad (4032)$$

$$\tau^5_{\gamma,\alpha} = \sum_{a \in V} W^4_{a,\alpha} Y^1_{a,\gamma} \quad (2r_T r_V N_v) \quad (4020)$$

$$\tau^5_{\gamma,\alpha,w} = \sum_{\delta \in A} \sum_{i \in O} {}^2D^4_{i,w} Y^{4,*}_{i,\gamma} \tau^2_{\delta,\alpha} \tau^1_{\delta,\gamma,w} \tau^4_{\delta,\alpha,i} \quad (5r_D r_T^2 r_V N_o) \quad (4033)$$

$$\tau^6_{\gamma,\alpha,i} = \sum_{\beta \in B} X_{\alpha,\beta} W^3_{i,\beta} \tau^5_{\gamma,\beta} \quad (3r_T r_V^2 N_o) \quad (4021)$$

$$\tau^6_{\gamma,\alpha,w} = \sum_{\beta \in B} X_{\alpha,\beta} \tau^5_{\gamma,\beta,w} \quad (2r_D r_T r_V^2) \quad (4034)$$

$$\tau_{\gamma,\alpha,w}^7 = \sum_{\delta \in A} Z_{\gamma,\delta}^* \tau_{\delta,\alpha,w}^6 \quad (2r_D r_T^2 r_V) \quad (4035)$$

$$\tau_{\alpha,i}^8 = \sum_{a \in V} {}^1T_{a,i} W_{a,\alpha}^2 \quad (2r_V N_o N_v) \quad (4036)$$

$$\tau_{\gamma,w,i}^9 = \sum_{\alpha \in B} \tau_{\alpha,i}^8 \tau_{\gamma,\alpha,w}^0 \tau_{\gamma,\alpha,w}^7 \quad (3r_D r_T r_V N_o) \quad (4037)$$

$${}^2R_{i,\gamma}^2 \leftarrow - \sum_{w \in D} \frac{1}{2} {}^2D_{i,w}^2 \tau_{\gamma,w,i}^9 \quad (2r_D r_T N_o) \quad (4038)$$

Raw expression

$${}^2R_{i,\epsilon}^2 \leftarrow \sum_{\gamma \in A} \sum_{j \in O} \sum_{k \in O} \sum_{l \in O} \sum_{a \in V} \sum_{b \in V} \sum_{c \in V} \frac{1}{2} {}^1T_{c,i} Y_{a,\epsilon}^{1,*} Z_{\epsilon,\gamma}^* Y_{b,\gamma}^{3,*} Y_{j,\gamma}^{4,*} {}^2D_{a,i,b,j} {}^2T_{b,k,a,l} V_{l,c,k,j} \quad (4039)$$

Factorized expression

$$\tau_{\gamma,\alpha,w}^0 = \sum_{a \in V} {}^2D_{a,w}^1 W_{a,\alpha}^1 Y_{a,\gamma}^{1,*} \quad (3r_D r_T r_V N_v) \quad (4040)$$

$$\tau_{\gamma,\delta,w}^1 = \sum_{a \in V} {}^2D_{a,w}^3 Y_{a,\gamma}^3 Y_{a,\delta}^{3,*} \quad (3r_D r_T^2 N_v) \quad (4041)$$

$$\tau_{\gamma,\alpha}^2 = \sum_{a \in V} W_{a,\alpha}^4 Y_{a,\gamma}^1 \quad (2r_T r_V N_v) \quad (4042)$$

$$\tau_{\gamma,\alpha,i}^3 = \sum_{\delta \in A} Y_{i,\delta}^2 Z_{\delta,\gamma} \tau_{\delta,\alpha}^2 \quad (3r_T^2 r_V N_o) \quad (4043)$$

$$\tau_{\gamma,\alpha}^4 = \sum_{i \in O} W_{i,\alpha}^3 Y_{i,\gamma}^4 \quad (2r_T r_V N_o) \quad (4044)$$

$$\tau_{\gamma,\alpha,w}^5 = \sum_{\delta \in A} \sum_{i \in O} {}^2D_{i,w}^4 Y_{i,\gamma}^{4,*} \tau_{\delta,\alpha}^4 \tau_{\delta,\gamma,w}^1 \tau_{\delta,\alpha,i}^3 \quad (5r_D r_T^2 r_V N_o) \quad (4045)$$

$$\tau_{\gamma,\alpha,w}^6 = \sum_{\beta \in B} X_{\alpha,\beta} \tau_{\gamma,\beta,w}^5 \quad (2r_D r_T r_V^2) \quad (4046)$$

$$\tau_{\gamma,\alpha,w}^7 = \sum_{\delta \in A} Z_{\gamma,\delta}^* \tau_{\delta,\alpha,w}^6 \quad (2r_D r_T^2 r_V) \quad (4047)$$

$$\tau_{\alpha,i}^8 = \sum_{a \in V} {}^1T_{a,i} W_{a,\alpha}^2 \quad (2r_V N_o N_v) \quad (4048)$$

$$\tau_{\gamma,w,i}^9 = \sum_{\alpha \in B} \tau_{\alpha,i}^8 \tau_{\gamma,\alpha,w}^0 \tau_{\gamma,\alpha,w}^7 \quad (3r_D r_T r_V N_o) \quad (4049)$$

$${}^2R_{i,\gamma}^2 \leftarrow - \sum_{w \in D} \frac{1}{2} {}^2D_{i,w}^2 \tau_{\gamma,w,i}^9 \quad (2r_D r_T N_o) \quad (4050)$$

Raw expression

$${}^2R_{i,\epsilon}^2 \leftarrow \sum_{\gamma \in A} \sum_{j \in O} \sum_{k \in O} \sum_{l \in O} \sum_{a \in V} \sum_{b \in V} \sum_{c \in V} \frac{1}{2} {}^1T_{c,j} Y_{a,\epsilon}^{1,*} Z_{\epsilon,\gamma}^* Y_{b,\gamma}^{3,*} Y_{j,\gamma}^{4,*} {}^2D_{a,i,b,j} {}^2T_{a,k,b,l} V_{k,i,l,c} \quad (4051)$$

Factorized expression

$$\tau_{\alpha,i}^0 = \sum_{a \in V} {}^1T_{a,i} W_{a,\alpha}^4 \quad (2r_V N_o N_v) \quad (4052)$$

$$\tau_{\alpha,i,j}^1 = \sum_{\beta \in B} X_{\alpha,\beta} W_{j,\beta}^3 \tau_{\beta,i}^0 \quad (3r_V^2 N_o^2) \quad (4053)$$

$$\tau_{\gamma,\alpha,i}^2 = \sum_{j \in O} Y_{j,\gamma}^4 \tau_{\alpha,i,j}^1 \quad (2r_T r_V N_o^2) \quad (4054)$$

$$\tau_{\gamma,\alpha}^3 = \sum_{a \in V} W_{a,\alpha}^2 Y_{a,\gamma}^3 \quad (2r_T r_V N_v) \quad (4055)$$

$$\tau_{\gamma,i,a}^4 = \sum_{\alpha \in B} W_{a,\alpha}^1 \tau_{\gamma,\alpha}^3 \tau_{\gamma,\alpha,i}^2 \quad (3r_T r_V N_o N_v) \quad (4056)$$

$$\tau_{\gamma,\delta,w}^5 = \sum_{a \in V} {}^2D_{a,w}^3 Y_{a,\gamma}^1 Y_{a,\delta}^{3,*} \quad (3r_D r_T^2 N_v) \quad (4057)$$

$$\tau_{\gamma,\delta,w}^6 = \sum_{i \in O} {}^2D_{i,w}^4 Y_{i,\gamma}^2 Y_{i,\delta}^{4,*} \quad (3r_D r_T^2 N_o) \quad (4058)$$

$$\tau_{\gamma,\delta,w}^7 = \sum_{\epsilon \in A} Z_{\delta,\epsilon}^* \tau_{\gamma,\epsilon,w}^5 \tau_{\gamma,\epsilon,w}^6 \quad (3r_D r_T^3) \quad (4059)$$

$$\tau_{\gamma,\delta,w}^8 = \sum_{\epsilon \in A} Z_{\epsilon,\gamma} \tau_{\epsilon,\delta,w}^7 \quad (2r_D r_T^3) \quad (4060)$$



$$\tau_{\gamma,i,a}^9 = \sum_{\delta \in A} \sum_{w \in D} {}^2D_{a,w}^1 {}^2D_{i,w}^2 \tau_{\delta,i,a}^4 \tau_{\delta,\gamma,w}^8 \quad (4r_D r_T^2 N_o N_v) \quad {}^2R_{i,\gamma}^2 \leftarrow - \sum_{a \in V} \frac{1}{2} Y_{a,\gamma}^{1,*} \tau_{\gamma,i,a}^9 \quad (2r_T N_o N_v) \quad (4074)$$

(4061)

Raw expression

$${}^2R_{i,\gamma}^2 \leftarrow - \sum_{a \in V} \frac{1}{2} Y_{a,\gamma}^{1,*} \tau_{\gamma,i,a}^9 \quad (2r_T N_o N_v) \quad (4062)$$

$${}^2R_{i,\epsilon}^2 \leftarrow \sum_{\gamma \in A} \sum_{j \in O} \sum_{k \in O} \sum_{l \in O} \sum_{a \in V} \sum_{b \in V} \sum_{c \in V} \frac{1}{2} {}^1T_{c,k} Y_{a,\epsilon}^{1,*} Z_{\epsilon,\gamma}^{*,*} Y_{b,\gamma}^{3,*} Y_{j,\gamma}^{4,*} {}^2D_{a,i,b,j} {}^2T_{a,i,b,l} V_{l,c,k,j} \quad (4075)$$

Raw expression

$${}^2R_{i,\epsilon}^2 \leftarrow \sum_{\gamma \in A} \sum_{j \in O} \sum_{k \in O} \sum_{l \in O} \sum_{a \in V} \sum_{b \in V} \sum_{c \in V} \frac{1}{2} {}^1T_{c,j} Y_{a,\epsilon}^{1,*} Z_{\epsilon,\gamma}^{*,*} Y_{b,\gamma}^{3,*} Y_{j,\gamma}^{4,*} {}^2D_{a,i,b,j} {}^2T_{b,k,a,l} V_{l,i,k,c} \quad (4063)$$

Factorized expression

$$\tau_{\gamma,\delta,w}^0 = \sum_{a \in V} {}^2D_{a,w}^1 Y_{a,\gamma}^1 Y_{a,\delta}^{1,*} \quad (3r_D r_T^2 N_v) \quad (4076)$$

Factorized expression

$$\tau_{\alpha,i}^0 = \sum_{a \in V} {}^1T_{a,i} W_{a,\alpha}^4 \quad (2r_V N_o N_v) \quad (4064)$$

$$\tau_{\gamma,\alpha,w}^1 = \sum_{a \in V} {}^2D_{a,w}^3 W_{a,\alpha}^1 Y_{a,\gamma}^{3,*} \quad (3r_D r_T r_V N_v) \quad (4077)$$

$$\tau_{\alpha,i,j}^1 = \sum_{\beta \in B} X_{\alpha,\beta} W_{j,\beta}^3 \tau_{\beta,i}^0 \quad (3r_V^2 N_o^2) \quad (4065)$$

$$\tau_{\gamma,\alpha}^2 = \sum_{a \in V} W_{a,\alpha}^2 Y_{a,\gamma}^3 \quad (2r_T r_V N_v) \quad (4078)$$

$$\tau_{\gamma,\alpha,i}^2 = \sum_{j \in O} Y_{j,\gamma}^2 \tau_{\alpha,i,j}^1 \quad (2r_T r_V N_o^2) \quad (4066)$$

$$\tau_{\gamma,\alpha,i}^3 = \sum_{\delta \in A} Z_{\gamma,\delta} Y_{i,\delta}^4 \tau_{\delta,\alpha}^2 \quad (3r_T^2 r_V N_o) \quad (4079)$$

$$\tau_{\gamma,\alpha}^3 = \sum_{a \in V} W_{a,\alpha}^2 Y_{a,\gamma}^1 \quad (2r_T r_V N_v) \quad (4067)$$

$$\tau_{\gamma,\delta,\alpha,w}^4 = \sum_{i \in O} {}^2D_{i,w}^4 Y_{i,\delta}^{4,*} \tau_{\delta,\alpha,w}^1 \tau_{\gamma,\alpha,i}^3 \quad (4r_D r_T^2 r_V N_o) \quad (4080)$$

$$\tau_{\gamma,i,a}^4 = \sum_{\alpha \in B} W_{a,\alpha}^1 \tau_{\gamma,\alpha}^3 \tau_{\gamma,\alpha,i}^2 \quad (3r_T r_V N_o N_v) \quad (4068)$$

$$\tau_{\alpha,i}^5 = \sum_{a \in V} {}^1T_{a,i} W_{a,\alpha}^4 \quad (2r_V N_o N_v) \quad (4081)$$

$$\tau_{\gamma,\delta,w}^5 = \sum_{a \in V} {}^2D_{a,w}^3 Y_{a,\gamma}^3 Y_{a,\delta}^{3,*} \quad (3r_D r_T^2 N_v) \quad (4069)$$

$$\tau_{\alpha,i,j}^6 = \sum_{\beta \in B} X_{\alpha,\beta} W_{j,\beta}^3 \tau_{\beta,i}^5 \quad (3r_V^2 N_o^2) \quad (4082)$$

$$\tau_{\gamma,\delta,w}^6 = \sum_{i \in O} {}^2D_{i,w}^4 Y_{i,\gamma}^4 Y_{i,\delta}^{4,*} \quad (3r_D r_T^2 N_o) \quad (4070)$$

$$\tau_{\gamma,\alpha,i}^7 = \sum_{j \in O} Y_{j,\gamma}^2 \tau_{\alpha,i,j}^6 \quad (2r_T r_V N_o^2) \quad (4083)$$

$$\tau_{\gamma,\delta,w}^7 = \sum_{\epsilon \in A} Z_{\gamma,\epsilon}^* \tau_{\gamma,\epsilon,w}^5 \tau_{\gamma,\epsilon,w}^6 \quad (3r_D r_T^3) \quad (4071)$$

$$\tau_{\gamma,\delta,w,i}^8 = \sum_{\alpha \in B} \tau_{\gamma,\alpha,i}^7 \tau_{\gamma,\delta,\alpha,w}^4 \quad (2r_D r_T^2 r_V N_o) \quad (4084)$$

$$\tau_{\gamma,\delta,w}^8 = \sum_{\epsilon \in A} Z_{\gamma,\epsilon} \tau_{\epsilon,\delta,w}^7 \quad (2r_D r_T^3) \quad (4072)$$

$$\tau_{\gamma,\delta,i}^9 = \sum_{\epsilon \in A} \sum_{w \in D} {}^2D_{i,w}^2 \tau_{\epsilon,\gamma,w}^0 \tau_{\epsilon,\delta,w,i}^8 \quad (3r_D r_T^3 N_o) \quad (4085)$$

$$\tau_{\gamma,i,a}^9 = \sum_{\delta \in A} \sum_{w \in D} {}^2D_{a,w}^1 {}^2D_{i,w}^2 \tau_{\delta,i,a}^4 \tau_{\delta,\gamma,w}^8 \quad (4r_D r_T^2 N_o N_v) \quad (4073)$$

$${}^2R_{i,\gamma}^2 \leftarrow - \sum_{\delta \in A} \frac{1}{2} Z_{\gamma,\delta}^* \tau_{\gamma,\delta,i}^9 \quad (2r_T^2 N_o) \quad (4086)$$

Raw expression

$${}^2R^2_{i,\epsilon} \leftarrow \sum_{\gamma \in A} \sum_{j \in O} \sum_{k \in O} \sum_{l \in O} \sum_{a \in V} \sum_{b \in V} \sum_{c \in V} \frac{1}{2} {}^1T_{c,k} Y^{1,*}_{a,\epsilon} Z^*_{\epsilon,\gamma} Y^{3,*}_{b,\gamma} Y^{4,*}_{j,\gamma} {}^2D^{a,i,b,j} {}^2T_{a,l,b,j} V_{k,i,l,c} \quad (4087)$$

Factorized expression

$$\tau^0_{\gamma,\delta,w} = \sum_{a \in V} {}^2D^1_{a,w} Y^3_{a,\gamma} Y^{1,*}_{a,\delta} (3r_D r_T^2 N_v) \quad (4088)$$

$$\tau^1_{\gamma,\alpha,w} = \sum_{a \in V} {}^2D^3_{a,w} W^1_{a,\alpha} Y^{3,*}_{a,\gamma} (3r_D r_T r_V N_v) \quad (4089)$$

$$\tau^2_{\gamma,\alpha} = \sum_{a \in V} W^2_{a,\alpha} Y^1_{a,\gamma} (2r_T r_V N_v) \quad (4090)$$

$$\tau^3_{\gamma,\alpha,i} = \sum_{\delta \in A} Y^2_{i,\delta} Z_{\delta,\gamma} \tau^2_{\delta,\alpha} (3r_T^2 r_V N_o) \quad (4091)$$

$$\tau^4_{\gamma,\delta,\alpha,w} = \sum_{i \in O} {}^2D^4_{i,w} Y^{4,*}_{i,\delta} \tau^1_{\delta,\alpha,w} \tau^3_{\gamma,\alpha,i} (4r_D r_T^2 r_V N_o) \quad (4092)$$

$$\tau^5_{\alpha,i} = \sum_{a \in V} {}^1T_{a,i} W^4_{a,\alpha} (2r_V N_o N_v) \quad (4093)$$

$$\tau^6_{\alpha,i,j} = \sum_{\beta \in B} X_{\alpha,\beta} W^3_{j,\beta} \tau^5_{\beta,i} (3r_V^2 N_o^2) \quad (4094)$$

$$\tau^7_{\gamma,\alpha,i} = \sum_{j \in O} Y^4_{j,\gamma} \tau^6_{\alpha,i,j} (2r_T r_V N_o^2) \quad (4095)$$

$$\tau^8_{\gamma,\delta,w,i} = \sum_{\alpha \in B} \tau^7_{\gamma,\alpha,i} \tau^4_{\gamma,\delta,\alpha,w} (2r_D r_T^2 r_V N_o) \quad (4096)$$

$$\tau^9_{\gamma,\delta,i} = \sum_{\epsilon \in A} \sum_{w \in D} {}^2D^2_{i,w} \tau^0_{\epsilon,\gamma,w} \tau^8_{\epsilon,\delta,w,i} (3r_D r_T^3 N_o) \quad (4097)$$

$${}^2R^2_{i,\gamma} \leftarrow - \sum_{\delta \in A} \frac{1}{2} Z^*_{\gamma,\delta} \tau^9_{\gamma,\delta,i} (2r_T^2 N_o) \quad (4098)$$

Raw expression

$${}^2R^2_{i,\epsilon} \leftarrow \sum_{\gamma \in A} \sum_{j \in O} \sum_{k \in O} \sum_{l \in O} \sum_{a \in V} \sum_{b \in V} \sum_{c \in V} \frac{1}{2} {}^1T_{c,k} Y^{1,*}_{a,\epsilon} Z^*_{\epsilon,\gamma} Y^{3,*}_{b,\gamma} Y^{4,*}_{j,\gamma} {}^2D^{a,i,b,j} {}^2T_{b,j,a,l} V_{k,i,l,c} \quad (4099)$$

Factorized expression

$$\tau^0_{\gamma,\alpha,w} = \sum_{a \in V} {}^2D^1_{a,w} W^1_{a,\alpha} Y^{1,*}_{a,\gamma} (3r_D r_T r_V N_v) \quad (4100)$$

$$\tau^1_{\gamma,\alpha} = \sum_{a \in V} W^2_{a,\alpha} Y^3_{a,\gamma} (2r_T r_V N_v) \quad (4101)$$

$$\tau^2_{\gamma,\alpha,i} = \sum_{\delta \in A} Z_{\gamma,\delta} Y^4_{i,\delta} \tau^1_{\delta,\alpha} (3r_T^2 r_V N_o) \quad (4102)$$

$$\tau^3_{\gamma,\delta,w} = \sum_{a \in V} {}^2D^3_{a,w} Y^1_{a,\gamma} Y^{3,*}_{a,\delta} (3r_D r_T^2 N_v) \quad (4103)$$

$$\tau^4_{\gamma,\delta,w,i} = \sum_{\epsilon \in A} {}^2D^4_{i,w} Z^*_{\delta,\epsilon} Y^{4,*}_{i,\epsilon} \tau^3_{\gamma,\epsilon,w} (4r_D r_T^3 N_o) \quad (4104)$$

$$\tau^5_{\alpha,i} = \sum_{a \in V} {}^1T_{a,i} W^4_{a,\alpha} (2r_V N_o N_v) \quad (4105)$$

$$\tau^6_{\alpha,i,j} = \sum_{\beta \in B} X_{\alpha,\beta} W^3_{j,\beta} \tau^5_{\beta,i} (3r_V^2 N_o^2) \quad (4106)$$

$$\tau^7_{\gamma,\alpha,i} = \sum_{j \in O} Y^2_{j,\gamma} \tau^6_{\alpha,i,j} (2r_T r_V N_o^2) \quad (4107)$$

$$\tau^8_{\gamma,\delta,\alpha,w} = \sum_{i \in O} \tau^7_{\gamma,\alpha,i} \tau^4_{\gamma,\delta,w,i} (2r_D r_T^2 r_V N_o) \quad (4108)$$

$$\tau^9_{\gamma,\alpha,w,i} = \sum_{\delta \in A} \tau^2_{\delta,\alpha,i} \tau^8_{\delta,\gamma,\alpha,w} (2r_D r_T^2 r_V N_o) \quad (4109)$$

$$\tau^{10}_{\gamma,w,i} = \sum_{\alpha \in B} \tau^0_{\gamma,\alpha,w} \tau^9_{\gamma,\alpha,w,i} (2r_D r_T r_V N_o) \quad (4110)$$

$${}^2R^2_{i,\gamma} \leftarrow - \sum_{w \in D} \frac{1}{2} {}^2D^2_{i,w} \tau^{10}_{\gamma,w,i} (2r_D r_T N_o) \quad (4111)$$

Raw expression

$${}^2R^2_{i,\epsilon} \leftarrow \sum_{\gamma \in A} \sum_{j \in O} \sum_{k \in O} \sum_{l \in O} \sum_{a \in V} \sum_{b \in V} \sum_{c \in V} \frac{1}{2} {}^1T_{c,k} Y^{1,*}_{a,\epsilon} Z^*_{\epsilon,\gamma} Y^{3,*}_{b,\gamma} Y^{4,*}_{j,\gamma} {}^2D^{a,i,b,j} {}^2T_{b,l,a,i} V_{l,c,k,j} \quad (4112)$$

Factorized expression

$$\tau^0_{\gamma,\alpha,w} = \sum_{a \in V} {}^2D^1_{a,w} W^1_{a,\alpha} Y^{1,*}_{a,\gamma} (3r_D r_T r_V N_v) \quad (4113)$$

$$\tau^1_{\gamma,\alpha} = \sum_{a \in V} W^2_{a,\alpha} Y^1_{a,\gamma} (2r_T r_V N_v) \quad (4114)$$

$$\tau^2_{\gamma,\alpha,i} = \sum_{\delta \in A} Y^2_{i,\delta} Z_{\delta,\gamma} \tau^1_{\delta,\alpha} (3r_T^2 r_V N_o) \quad (4115)$$

$$\tau^3_{\gamma,\delta,w} = \sum_{a \in V} {}^2D^3_{a,w} Y^3_{a,\gamma} Y^{3,*}_{a,\delta} (3r_D r_T^2 N_v) \quad (4116)$$

$$\tau^4_{\gamma,\delta,w,i} = \sum_{\epsilon \in A} {}^2D^4_{i,w} Z^*_{\delta,\epsilon} Y^{4,*}_{i,\epsilon} \tau^3_{\gamma,\epsilon,w} (4r_D r_T^3 N_o) \quad (4117)$$

$$\tau^5_{\alpha,i} = \sum_{a \in V} {}^1T_{a,i} W^4_{a,\alpha} (2r_V N_o N_v) \quad (4118)$$

$$\tau^6_{\alpha,i,j} = \sum_{\beta \in B} X_{\alpha,\beta} W^3_{j,\beta} \tau^5_{\beta,i} (3r_V^2 N_o^2) \quad (4119)$$

$$\tau^7_{\gamma,\alpha,i} = \sum_{j \in O} Y^4_{j,\gamma} \tau^6_{\alpha,i,j} (2r_T r_V N_o^2) \quad (4120)$$

$$\tau^8_{\gamma,\delta,\alpha,w} = \sum_{i \in O} \tau^7_{\gamma,\alpha,i} \tau^4_{\gamma,\delta,w,i} (2r_D r_T^2 r_V N_o) \quad (4121)$$

$$\tau^9_{\gamma,\alpha,w,i} = \sum_{\delta \in A} \tau^2_{\delta,\alpha,i} \tau^8_{\delta,\gamma,\alpha,w} (2r_D r_T^2 r_V N_o) \quad (4122)$$

$$\tau^{10}_{\gamma,w,i} = \sum_{\alpha \in B} \tau^0_{\gamma,\alpha,w} \tau^9_{\gamma,\alpha,w,i} (2r_D r_T r_V N_o) \quad (4123)$$

$${}^2R^2_{i,\gamma} \leftarrow - \sum_{w \in D} \frac{1}{2} {}^2D^2_{i,w} \tau^{10}_{\gamma,w,i} (2r_D r_T N_o) \quad (4124)$$

Raw expression

$${}^2R^2_{i,\epsilon} \leftarrow - \sum_{\gamma \in A} \sum_{j \in O} \sum_{k \in O} \sum_{l \in O} \sum_{a \in V} \sum_{b \in V} \sum_{c \in V} {}^1T_{a,k} Y^{1,*}_{a,\epsilon} Z^*_{\epsilon,\gamma} Y^{3,*}_{b,\gamma} Y^{4,*}_{j,\gamma} {}^2D^{a,i,b,j} {}^2T_{b,j,c,l} V_{k,i,l,c} \quad (4125)$$

Factorized expression

$$\tau^0_{\gamma,\delta,w} = \sum_{a \in V} {}^2D^1_{a,w} Y^1_{a,\gamma} Y^{1,*}_{a,\delta} (3r_D r_T^2 N_v) \quad (4126)$$

$$\tau^1_{\gamma,\alpha} = \sum_{i \in O} W^3_{i,\alpha} Y^2_{i,\gamma} (2r_T r_V N_o) \quad (4127)$$

$$\tau^2_{\gamma,\alpha} = \sum_{a \in V} W^4_{a,\alpha} Y^3_{a,\gamma} (2r_T r_V N_v) \quad (4128)$$

$$\tau^3_{\gamma,\alpha,i} = \sum_{\delta \in A} Z_{\gamma,\delta} Y^4_{i,\delta} \tau^2_{\delta,\alpha} (3r_T^2 r_V N_o) \quad (4129)$$

$$\tau^4_{\alpha,i} = \sum_{a \in V} {}^1T_{a,i} W^2_{a,\alpha} (2r_V N_o N_v) \quad (4130)$$

$$\tau^5_{\gamma,\alpha,w} = \sum_{i \in O} {}^2D^4_{i,w} Y^{4,*}_{i,\gamma} \tau^4_{\alpha,i} (3r_D r_T r_V N_o) \quad (4131)$$

$$\tau^6_{\gamma,\alpha,w} = \sum_{a \in V} {}^2D^3_{a,w} W^1_{a,\alpha} Y^{3,*}_{a,\gamma} (3r_D r_T r_V N_v) \quad (4132)$$

$$\tau^7_{\gamma,\alpha,w} = \sum_{\beta \in B} X_{\beta,\alpha} \tau^5_{\gamma,\beta,w} \tau^6_{\gamma,\beta,w} (3r_D r_T r_V^2) \quad (4133)$$

$$\tau^8_{\gamma,\alpha,w} = \sum_{\delta \in A} Z^*_{\gamma,\delta} \tau^7_{\delta,\alpha,w} (2r_D r_T^2 r_V) \quad (4134)$$

$$\tau^9_{\gamma,\delta,w,i} = \sum_{\alpha \in B} \tau^1_{\gamma,\alpha} \tau^3_{\gamma,\alpha,i} \tau^8_{\delta,\alpha,w} (3r_D r_T^2 r_V N_o) \quad (4135)$$

$$\tau^{10}_{\gamma,w,i} = \sum_{\delta \in A} \tau^0_{\delta,\gamma,w} \tau^9_{\delta,\gamma,w,i} (2r_D r_T^2 N_o) \quad (4136)$$

$${}^2R^2_{i,\gamma} \leftarrow - \sum_{w \in D} \frac{1}{2} {}^2D^2_{i,w} \tau^{10}_{\gamma,w,i} (2r_D r_T N_o) \quad (4137)$$

Raw expression

$${}^2R^2_{i,\epsilon} \leftarrow - \sum_{\gamma \in A} \sum_{j \in O} \sum_{k \in O} \sum_{l \in O} \sum_{a \in V} \sum_{b \in V} \sum_{c \in V} {}^1T_{a,k} Y^{1,*}_{a,\epsilon} Z^*_{\epsilon,\gamma} Y^{3,*}_{b,\gamma} Y^{4,*}_{j,\gamma} {}^2D^{a,i,b,j} {}^2T_{c,l,b,j} V_{k,i,l,c} \quad (4138)$$

Factorized expression

$$\tau^0_{\gamma,\delta,w} = \sum_{a \in V} {}^2D^1_{a,w} Y^3_{a,\gamma} Y^{1,*}_{a,\delta} (3r_D r_T^2 N_v) \quad (4139)$$

$$\tau^1_{\gamma,\alpha} = \sum_{a \in V} W^4_{a,\alpha} Y^1_{a,\gamma} (2r_T r_V N_v) \quad (4140)$$

$$\tau^2_{\gamma,\alpha,i} = \sum_{\delta \in A} Y^2_{i,\delta} Z_{\delta,\gamma} \tau^1_{\delta,\alpha} (3r_T^2 r_V N_o) \quad (4141)$$

$$\tau^3_{\gamma,\alpha} = \sum_{i \in O} W^3_{i,\alpha} Y^4_{i,\gamma} (2r_T r_V N_o) \quad (4142)$$

$$\tau^4_{\alpha,i} = \sum_{a \in V} {}^1T_{a,i} W^2_{a,\alpha} (2r_V N_o N_v) \quad (4143)$$

$$\tau^5_{\gamma,\alpha,w} = \sum_{i \in O} {}^2D^4_{i,w} Y^{4,*}_{i,\gamma} \tau^4_{\alpha,i} (3r_D r_T r_V N_o) \quad (4144)$$

$$\tau^6_{\gamma,\alpha,w} = \sum_{a \in V} {}^2D^3_{a,w} W^1_{a,\alpha} Y^{3,*}_{a,\gamma} (3r_D r_T r_V N_v) \quad (4145)$$

$$\tau^7_{\gamma,\alpha,w} = \sum_{\beta \in B} X_{\beta,\alpha} \tau^5_{\gamma,\beta,w} \tau^6_{\gamma,\beta,w} (3r_D r_T r_V^2) \quad (4146)$$

$$\tau^8_{\gamma,\alpha,w} = \sum_{\delta \in A} Z^*_{\gamma,\delta} \tau^7_{\delta,\alpha,w} (2r_D r_T^2 r_V) \quad (4147)$$

$$\tau^9_{\gamma,\delta,w,i} = \sum_{\alpha \in B} \tau^3_{\gamma,\alpha} \tau^2_{\gamma,\alpha,i} \tau^8_{\delta,\alpha,w} (3r_D r_T^2 r_V N_o) \quad (4148)$$

$$\tau^{10}_{\gamma,w,i} = \sum_{\delta \in A} \tau^0_{\delta,\gamma,w} \tau^9_{\delta,\gamma,w,i} (2r_D r_T^2 N_o) \quad (4149)$$

$${}^2R^2_{i,\gamma} \leftarrow - \sum_{w \in D} \frac{1}{2} {}^2D^2_{i,w} \tau^{10}_{\gamma,w,i} (2r_D r_T N_o) \quad (4150)$$

Raw expression

$${}^2R^2_{i,\epsilon} \leftarrow - \sum_{\gamma \in A} \sum_{j \in O} \sum_{k \in O} \sum_{l \in O} \sum_{a \in V} \sum_{b \in V} \sum_{c \in V} {}^1T_{b,k} Y^{1,*}_{a,\epsilon} Z^*_{\epsilon,\gamma} Y^{3,*}_{b,\gamma} Y^{4,*}_{j,\gamma} {}^2D^{a,i,b,j} {}^2T_{a,i,c,l} V_{l,c,k,j} \quad (4151)$$

Factorized expression

$$\tau^0_{\gamma,\delta,w} = \sum_{a \in V} {}^2D^1_{a,w} Y^1_{a,\gamma} Y^{1,*}_{a,\delta} (3r_D r_T^2 N_v) \quad (4152)$$

$$\tau^1_{\alpha,i} = \sum_{a \in V} {}^1T_{a,i} W^4_{a,\alpha} (2r_V N_o N_v) \quad (4153)$$

$$\tau^2_{\alpha,i,j} = \sum_{\beta \in B} X_{\alpha,\beta} W^3_{j,\beta} \tau^1_{\beta,i} (3r_V^2 N_o^2) \quad (4154)$$

$$\tau^3_{\gamma,\alpha,i} = \sum_{j \in O} Y^4_{j,\gamma} \tau^2_{\alpha,i,j} (2r_T r_V N_o^2) \quad (4155)$$

$$\tau^4_{\gamma,\alpha} = \sum_{a \in V} W^2_{a,\alpha} Y^3_{a,\gamma} (2r_T r_V N_v) \quad (4156)$$

$$\tau^5_{\gamma,i,a} = \sum_{\alpha \in B} W^1_{a,\alpha} \tau^4_{\gamma,\alpha} \tau^3_{\gamma,\alpha,i} (3r_T r_V N_o N_v) \quad (4157)$$

$$\tau^6_{\gamma,\delta,w} = \sum_{i \in O} \sum_{a \in V} {}^2D^3_{a,w} {}^2D^4_{i,w} Y^{3,*}_{a,\delta} Y^{4,*}_{i,\delta} \tau^5_{\gamma,i,a} (5r_D r_T^2 N_o N_v) \quad (4158)$$

$$\tau^7_{\gamma,\delta,w} = \sum_{\epsilon \in A} Z^*_{\delta,\epsilon} \tau^6_{\gamma,\epsilon,w} (2r_D r_T^3) \quad (4159)$$

$$\tau^8_{\gamma,\delta,w} = \sum_{\epsilon \in A} Z_{\gamma,\epsilon} \tau^7_{\epsilon,\delta,w} (2r_D r_T^3) \quad (4160)$$

$${}^2R^2_{i,\gamma} \leftarrow - \sum_{\delta \in A} \sum_{w \in D} \frac{1}{2} {}^2D^2_{i,w} Y^2_{i,\delta} \tau^0_{\delta,\gamma,w} \tau^8_{\delta,\gamma,w} (4r_D r_T^2 N_o) \quad (4161)$$

Raw expression

$${}^2R^2_{i,\epsilon} \leftarrow - \sum_{\gamma \in A} \sum_{j \in O} \sum_{k \in O} \sum_{l \in O} \sum_{a \in V} \sum_{b \in V} \sum_{c \in V} {}^1T_{b,k} Y^{1,*}_{a,\epsilon} Z^*_{\epsilon,\gamma} Y^{3,*}_{b,\gamma} Y^{4,*}_{j,\gamma} {}^2D^{a,i,b,j} {}^2T_{c,l,a,i} V_{l,c,k,j} \quad (4162)$$

Factorized expression

$$\tau_{\gamma,\delta,w}^0 = \sum_{a \in V} {}^2D_{a,w}^1 Y_{a,\gamma}^3 Y_{a,\delta}^{1,*} \quad (3r_D r_T^2 N_v) \quad (4163)$$

$$\tau_{\gamma,\delta,w}^2 = \sum_{\epsilon \in A} Z_{\delta,\epsilon}^* \tau_{\gamma,\epsilon,w}^0 \tau_{\gamma,\epsilon,w}^1 \quad (3r_D r_T^3) \quad (4176)$$

$$\tau_{\alpha,i}^1 = \sum_{a \in V} {}^1T_{a,i} W_{a,\alpha}^4 \quad (2r_V N_o N_v) \quad (4164)$$

$$\tau_{\gamma,\delta,w}^3 = \sum_{\epsilon \in A} Z_{\epsilon,\gamma} \tau_{\epsilon,\delta,w}^2 \quad (2r_D r_T^3) \quad (4177)$$

$$\tau_{\alpha,i,j}^2 = \sum_{\beta \in B} X_{\alpha,\beta} W_{j,\beta}^3 \tau_{\beta,i}^1 \quad (3r_V^2 N_o^2) \quad (4165)$$

$$\tau_{\alpha,i}^4 = \sum_{a \in V} {}^1T_{a,i} W_{a,\alpha}^2 \quad (2r_V N_o N_v) \quad (4178)$$

$$\tau_{\gamma,\alpha,i}^3 = \sum_{j \in O} Y_{j,\gamma}^2 \tau_{\alpha,i,j}^2 \quad (2r_T r_V N_o^2) \quad (4166)$$

$$\tau_{\alpha,\beta}^5 = \sum_{i \in O} W_{i,\beta}^3 \tau_{\alpha,i}^4 \quad (2r_V^2 N_o) \quad (4179)$$

$$\tau_{\gamma,\alpha}^4 = \sum_{a \in V} W_{a,\alpha}^2 Y_{a,\gamma}^1 \quad (2r_T r_V N_v) \quad (4167)$$

$$\tau_{\alpha,a}^6 = \sum_{\beta \in B} X_{\alpha,\beta} W_{a,\beta}^4 \tau_{\alpha,\beta}^5 \quad (3r_V^2 N_v) \quad (4180)$$

$$\tau_{\gamma,i,a}^5 = \sum_{\alpha \in B} W_{a,\alpha}^1 \tau_{\gamma,\alpha}^4 \tau_{\gamma,\alpha,i}^3 \quad (3r_T r_V N_o N_v) \quad (4168)$$

$$\tau_{a,b}^7 = \sum_{\alpha \in B} W_{a,\alpha}^1 \tau_{\alpha,b}^6 \quad (2r_V N_v^2) \quad (4181)$$

$$\tau_{\gamma,\delta,w}^6 = \sum_{i \in O} \sum_{a \in V} {}^2D_{a,w}^3 {}^2D_{i,w}^4 Y_{a,\delta}^{3,*} Y_{i,\delta}^{4,*} \tau_{\gamma,i,a}^5 \quad (5r_D r_T^2 N_o N_v) \quad (4169)$$

$$\tau_{\gamma,a}^8 = \sum_{b \in V} Y_{b,\gamma}^3 \tau_{a,b}^7 \quad (2r_T N_v^2) \quad (4182)$$

$$\tau_{\gamma,\delta,w}^7 = \sum_{\epsilon \in A} Z_{\delta,\epsilon}^* \tau_{\gamma,\epsilon,w}^6 \quad (2r_D r_T^3) \quad (4170)$$

$$\tau_{\gamma,\delta,w}^9 = \sum_{a \in V} {}^2D_{a,w}^1 Y_{a,\delta}^{1,*} \tau_{\gamma,a}^8 \quad (3r_D r_T^2 N_v) \quad (4183)$$

$$\tau_{\gamma,\delta,w}^8 = \sum_{\epsilon \in A} Z_{\epsilon,\gamma} \tau_{\epsilon,\delta,w}^7 \quad (2r_D r_T^3) \quad (4171)$$

$${}^2R_{i,\gamma}^2 \leftarrow - \sum_{\delta \in A} \sum_{w \in D} \frac{1}{2} {}^2D_{i,w}^2 Y_{i,\delta}^4 \tau_{\delta,\gamma,w}^0 \tau_{\delta,\gamma,w}^8 \quad (4r_D r_T^2 N_o) \quad (4184)$$

$${}^2R_{i,\gamma}^2 \leftarrow - \sum_{\delta \in A} \sum_{w \in D} \frac{1}{2} {}^2D_{i,w}^2 Y_{i,\delta}^4 \tau_{\delta,\gamma,w}^0 \tau_{\delta,\gamma,w}^8 \quad (4r_D r_T^2 N_o) \quad \text{Raw expression} \quad (4172)$$

Raw expression

$${}^2R_{i,\epsilon}^2 \leftarrow - \sum_{\gamma \in A} \sum_{j \in O} \sum_{k \in O} \sum_{l \in O} \sum_{a \in V} \sum_{b \in V} \sum_{c \in V} {}^1T_{c,k} Y_{a,\epsilon}^{1,*} Z_{\epsilon,\gamma}^* Y_{b,\gamma}^{3,*} Y_{j,\gamma}^{4,*} {}^2D_{a,i,b,j} {}^2T_{a,l,b,j} V_{l,i,k,c} \quad (4185)$$

$${}^2R_{i,\epsilon}^2 \leftarrow - \sum_{\gamma \in A} \sum_{j \in O} \sum_{k \in O} \sum_{l \in O} \sum_{a \in V} \sum_{b \in V} \sum_{c \in V} {}^1T_{c,k} Y_{a,\epsilon}^{1,*} Z_{\epsilon,\gamma}^* Y_{b,\gamma}^{3,*} Y_{j,\gamma}^{4,*} {}^2D_{a,i,b,j} {}^2T_{a,i,b,l} V_{k,c,l,j} \quad (4173)$$

Factorized expression

Factorized expression

$$\tau_{\gamma,\delta,w}^0 = \sum_{a \in V} {}^2D_{a,w}^3 Y_{a,\gamma}^1 Y_{a,\delta}^{3,*} \quad (3r_D r_T^2 N_v) \quad (4174)$$

$$\tau_{\gamma,\delta,w}^1 = \sum_{i \in O} {}^2D_{i,w}^4 Y_{i,\gamma}^4 Y_{i,\delta}^{4,*} \quad (3r_D r_T^2 N_o) \quad (4187)$$

$$\tau_{\gamma,\delta,w}^1 = \sum_{i \in O} {}^2D_{i,w}^4 Y_{i,\gamma}^2 Y_{i,\delta}^{4,*} \quad (3r_D r_T^2 N_o) \quad (4175)$$

$$\tau_{\gamma,\delta,w}^2 = \sum_{\epsilon \in A} Z_{\delta,\epsilon}^* \tau_{\gamma,\epsilon,w}^0 \tau_{\gamma,\epsilon,w}^1 \quad (3r_D r_T^3) \quad (4188)$$

$$\tau^3_{\gamma,\delta,w} = \sum_{\epsilon \in A} Z_{\gamma,\epsilon} \tau^2_{\epsilon,\delta,w} \quad (2r_D r_T^3) \quad (4189)$$

$$\tau^4_{\alpha,a} = \sum_{\beta \in B} X_{\alpha,\beta} W^4_{a,\beta} \tau^3_{\alpha,\beta} \quad (3r_V^2 N_v) \quad (4202)$$

$$\tau^4_{\alpha,i} = \sum_{a \in V} {}^1T_{a,i} W^2_{a,\alpha} \quad (2r_V N_o N_v) \quad (4190)$$

$$\tau^5_{a,b} = \sum_{\alpha \in B} W^1_{a,\alpha} \tau^4_{\alpha,b} \quad (2r_V N_v^2) \quad (4203)$$

$$\tau^5_{\alpha,\beta} = \sum_{i \in O} W^3_{i,\beta} \tau^4_{\alpha,i} \quad (2r_V^2 N_o) \quad (4191)$$

$$\tau^6_{\gamma,a} = \sum_{b \in V} Y^3_{b,\gamma} \tau^5_{a,b} \quad (2r_T N_v^2) \quad (4204)$$

$$\tau^6_{\alpha,a} = \sum_{\beta \in B} X_{\alpha,\beta} W^4_{a,\beta} \tau^5_{\alpha,\beta} \quad (3r_V^2 N_v) \quad (4192)$$

$$\tau^7_{\gamma,\delta,w} = \sum_{a \in V} {}^2D^3_{a,w} Y^{3,*}_{a,\delta} \tau^6_{\gamma,a} \quad (3r_D r_T^2 N_v) \quad (4205)$$

$$\tau^7_{a,b} = \sum_{\alpha \in B} W^1_{a,\alpha} \tau^6_{\alpha,b} \quad (2r_V N_v^2) \quad (4193)$$

$$\tau^8_{\gamma,\delta,w} = \sum_{\epsilon \in A} Z^*_{\delta,\epsilon} \tau^1_{\gamma,\epsilon,w} \tau^7_{\gamma,\epsilon,w} \quad (3r_D r_T^3) \quad (4206)$$

$$\tau^8_{\gamma,a} = \sum_{b \in V} Y^1_{b,\gamma} \tau^7_{a,b} \quad (2r_T N_v^2) \quad (4194)$$

$$\tau^9_{\gamma,\delta,w} = \sum_{\epsilon \in A} Z_{\gamma,\epsilon} \tau^8_{\epsilon,\delta,w} \quad (2r_D r_T^3) \quad (4207)$$

$$\tau^9_{\gamma,\delta,w} = \sum_{a \in V} {}^2D^1_{a,w} Y^{1,*}_{a,\delta} \tau^8_{\gamma,a} \quad (3r_D r_T^2 N_v) \quad (4195)$$

$${}^2R^2_{i,\gamma} \leftarrow - \sum_{\delta \in A} \sum_{w \in D} \frac{1}{2} {}^2D^2_{i,w} Y^2_{i,\delta} \tau^0_{\delta,\gamma,w} \tau^9_{\delta,\gamma,w} \quad (4r_D r_T^2 N_o) \quad (4208)$$

$${}^2R^2_{i,\gamma} \leftarrow - \sum_{\delta \in A} \sum_{w \in D} \frac{1}{2} {}^2D^2_{i,w} Y^2_{i,\delta} \tau^3_{\delta,\gamma,w} \tau^9_{\delta,\gamma,w} \quad (4r_D r_T^2 N_o) \quad \text{Raw expression} \quad (4196)$$

$${}^2R^2_{i,\epsilon} \leftarrow - \sum_{\gamma \in A} \sum_{j \in O} \sum_{k \in O} \sum_{l \in O} \sum_{a \in V} \sum_{b \in V} \sum_{c \in V} {}^1T_{c,k} Y^{1,*}_{a,\epsilon} Z^*_{\epsilon,\gamma} Y^{3,*}_{b,\gamma} Y^{4,*}_{j,\gamma} {}^2D^{a,i,b,j} {}^2T_{b,l,a,i} V_{k,c,l,j} \quad (4209)$$

Raw expression

$${}^2R^2_{i,\epsilon} \leftarrow - \sum_{\gamma \in A} \sum_{j \in O} \sum_{k \in O} \sum_{l \in O} \sum_{a \in V} \sum_{b \in V} \sum_{c \in V} {}^1T_{c,k} Y^{1,*}_{a,\epsilon} Z^*_{\epsilon,\gamma} Y^{3,*}_{b,\gamma} Y^{4,*}_{j,\gamma} {}^2D^{a,i,b,j} {}^2T_{b,j,a,l} V_{l,i,k,c} \quad (4197)$$

Factorized expression

$$\tau^0_{\gamma,\delta,w} = \sum_{i \in O} {}^2D^4_{i,w} Y^2_{i,\gamma} Y^{4,*}_{i,\delta} \quad (3r_D r_T^2 N_o) \quad (4210)$$

Factorized expression

$$\tau^0_{\gamma,\delta,w} = \sum_{a \in V} {}^2D^1_{a,w} Y^1_{a,\gamma} Y^{1,*}_{a,\delta} \quad (3r_D r_T^2 N_v) \quad (4198)$$

$$\tau^1_{\alpha,i} = \sum_{a \in V} {}^1T_{a,i} W^2_{a,\alpha} \quad (2r_V N_o N_v) \quad (4211)$$

$$\tau^1_{\gamma,\delta,w} = \sum_{i \in O} {}^2D^4_{i,w} Y^4_{i,\gamma} Y^{4,*}_{i,\delta} \quad (3r_D r_T^2 N_o) \quad (4199)$$

$$\tau^2_{\alpha,\beta} = \sum_{i \in O} W^3_{i,\beta} \tau^1_{\alpha,i} \quad (2r_V^2 N_o) \quad (4212)$$

$$\tau^2_{\alpha,i} = \sum_{a \in V} {}^1T_{a,i} W^2_{a,\alpha} \quad (2r_V N_o N_v) \quad (4200)$$

$$\tau^3_{\alpha,a} = \sum_{\beta \in B} X_{\alpha,\beta} W^4_{a,\beta} \tau^2_{\alpha,\beta} \quad (3r_V^2 N_v) \quad (4213)$$

$$\tau^3_{\alpha,\beta} = \sum_{i \in O} W^3_{i,\beta} \tau^2_{\alpha,i} \quad (2r_V^2 N_o) \quad (4201)$$

$$\tau^4_{a,b} = \sum_{\alpha \in B} W^1_{a,\alpha} \tau^3_{\alpha,b} \quad (2r_V N_v^2) \quad (4214)$$

$$\tau^5_{\gamma,a} = \sum_{b \in V} Y^1_{b,\gamma} \tau^4_{a,b} \quad (2r_T N_v^2) \quad (4215)$$

$$\tau^5_{\gamma,\alpha,w} = \sum_{\beta \in B} X_{\alpha,\beta} \tau^2_{\gamma,\beta,w} \tau^4_{\gamma,\beta,w} \quad (3r_D r_T r_V^2) \quad (4227)$$

$$\tau^6_{\gamma,\delta,w} = \sum_{a \in V} {}^2D^3_{a,w} Y^{3,*}_{a,\delta} \tau^5_{\gamma,a} \quad (3r_D r_T^2 N_v) \quad (4216)$$

$$\tau^6_{\gamma,\alpha,w} = \sum_{\delta \in A} Z^*_{\gamma,\delta} \tau^5_{\delta,\alpha,w} \quad (2r_D r_T^2 r_V) \quad (4228)$$

$$\tau^7_{\gamma,\delta,w} = \sum_{\epsilon \in A} Z^*_{\delta,\epsilon} \tau^0_{\gamma,\epsilon,w} \tau^6_{\gamma,\epsilon,w} \quad (3r_D r_T^3) \quad (4217)$$

$$\tau^7_{\gamma,w,i} = \sum_{a \in V} {}^2D^1_{a,w} {}^1T_{a,i} Y^{1,*}_{a,\gamma} \quad (3r_D r_T N_o N_v) \quad (4229)$$

$$\tau^8_{\gamma,\delta,w} = \sum_{\epsilon \in A} Z_{\epsilon,\gamma} \tau^7_{\epsilon,\delta,w} \quad (2r_D r_T^3) \quad (4218)$$

$$\tau^8_{\gamma,\alpha,w} = \sum_{i \in O} W^1_{i,\alpha} \tau^7_{\gamma,w,i} \quad (2r_D r_T r_V N_o) \quad (4230)$$

$$\tau^9_{\gamma,\delta,w} = \sum_{a \in V} {}^2D^1_{a,w} Y^3_{a,\gamma} Y^{1,*}_{a,\delta} \quad (3r_D r_T^2 N_v) \quad (4219)$$

$$\tau^9_{\gamma,w,i} = \sum_{\alpha \in B} \tau^0_{\alpha,i} \tau^6_{\gamma,\alpha,w} \tau^8_{\gamma,\alpha,w} \quad (3r_D r_T r_V N_o) \quad (4231)$$

$${}^2R^2_{i,\gamma} \leftarrow - \sum_{\delta \in A} \sum_{w \in D} \frac{1}{2} {}^2D^2_{i,w} Y^4_{i,\delta} \tau^8_{\delta,\gamma,w} \tau^9_{\delta,\gamma,w} \quad (4r_D r_T^2 N_o) \quad (4220)$$

$${}^2R^2_{i,\gamma} \leftarrow \sum_{w \in D} {}^2D^2_{i,w} \tau^9_{\gamma,w,i} \quad (2r_D r_T N_o) \quad (4232)$$

### G. Contributions from $(H^1 T^1 T^1 T^1 T)_c$

Raw expression

$${}^2R^2_{i,\epsilon} \leftarrow \sum_{\gamma \in A} \sum_{j \in O} \sum_{k \in O} \sum_{l \in O} \sum_{a \in V} \sum_{b \in V} \sum_{c \in V} \sum_{d \in V} {}^1T_{a,k} {}^1T_{b,l} {}^1T_{c,i} {}^1T_{d,j} Y^{1,*}_{a,\epsilon} Z^*_{\epsilon,\gamma} Y^{3,*}_{b,\gamma} Y^{4,*}_{j,\gamma} {}^2D^{a,i,b,j} V_{k,c,l,d} \quad (4221)$$

Factorized expression

$$\tau^0_{\alpha,i} = \sum_{a \in V} {}^1T_{a,i} W^2_{a,\alpha} \quad (2r_V N_o N_v) \quad (4222)$$

$$\tau^1_{\alpha,i} = \sum_{a \in V} {}^1T_{a,i} W^4_{a,\alpha} \quad (2r_V N_o N_v) \quad (4223)$$

$$\tau^2_{\gamma,\alpha,w} = \sum_{i \in O} {}^2D^4_{i,w} Y^{4,*}_{i,\gamma} \tau^1_{\alpha,i} \quad (3r_D r_T r_V N_o) \quad (4224)$$

$$\tau^3_{\gamma,w,i} = \sum_{a \in V} {}^2D^3_{a,w} {}^1T_{a,i} Y^{3,*}_{a,\gamma} \quad (3r_D r_T N_o N_v) \quad (4225)$$

$$\tau^4_{\gamma,\alpha,w} = \sum_{i \in O} W^3_{i,\alpha} \tau^3_{\gamma,w,i} \quad (2r_D r_T r_V N_o) \quad (4226)$$

### H. Contributions from $(H^1 T^1 T^2 T)_c$

Raw expression

$${}^2R^2_{i,\epsilon} \leftarrow \sum_{\gamma \in A} \sum_{j \in O} \sum_{k \in O} \sum_{l \in O} \sum_{a \in V} \sum_{b \in V} \sum_{c \in V} \sum_{d \in V} \frac{1}{2} {}^1T_{a,k} {}^1T_{b,l} Y^{1,*}_{a,\epsilon} Z^*_{\epsilon,\gamma} Y^{3,*}_{b,\gamma} Y^{4,*}_{j,\gamma} {}^2D^{a,i,b,j} {}^2T_{c,i,d,j} V_{k,c,l,d} \quad (4233)$$

Factorized expression

$$\tau^0_{\gamma,\alpha} = \sum_{a \in V} W^4_{a,\alpha} Y^3_{a,\gamma} \quad (2r_T r_V N_v) \quad (4234)$$

$$\tau^1_{\gamma,\alpha} = \sum_{i \in O} W^3_{i,\alpha} Y^4_{i,\gamma} \quad (2r_T r_V N_o) \quad (4235)$$

$$\tau^2_{\gamma,\alpha} = \sum_{\beta \in B} X_{\alpha,\beta} \tau^0_{\gamma,\beta} \tau^1_{\gamma,\beta} \quad (3r_T r_V^2) \quad (4236)$$

$$\tau^3_{\gamma,\alpha} = \sum_{\delta \in A} Z_{\gamma,\delta} \tau^2_{\delta,\alpha} \quad (2r_T^2 r_V) \quad (4237)$$

$$\tau^4_{\gamma,\delta,w} = \sum_{a \in V} {}^2D^3_{a,w} Y^1_{a,\gamma} Y^{3,*}_{a,\delta} \quad (3r_D r_T^2 N_v) \quad (4238)$$

$$\tau_{\gamma,\delta,w}^5 = \sum_{i \in O} {}^2D_{i,w}^4 Y_{i,\gamma}^2 Y_{i,\delta}^{4,*} \quad (3r_D r_T^2 N_o) \quad (4239)$$

$$\tau_{\gamma,\delta,w}^6 = \sum_{\epsilon \in A} Z_{\delta,\epsilon}^* \tau_{\gamma,\epsilon,w}^4 \tau_{\gamma,\epsilon,w}^5 \quad (3r_D r_T^3) \quad (4240)$$

$$\tau_{\gamma,\alpha,w}^7 = \sum_{\delta \in A} \tau_{\delta,\alpha}^3 \tau_{\delta,\gamma,w}^6 \quad (2r_D r_T^2 r_V) \quad (4241)$$

$$\tau_{\gamma,w,i}^8 = \sum_{a \in V} {}^2D_{a,w}^1 {}^1T_{a,i} Y_{a,\gamma}^{1,*} \quad (3r_D r_T N_o N_v) \quad (4242)$$

$$\tau_{\gamma,\alpha,w}^9 = \sum_{i \in O} W_{i,\alpha}^1 \tau_{\gamma,w,i}^8 \quad (2r_D r_T r_V N_o) \quad (4243)$$

$$\tau_{\alpha,i}^{10} = \sum_{a \in V} {}^1T_{a,i} W_{a,\alpha}^2 \quad (2r_V N_o N_v) \quad (4244)$$

$$\tau_{\gamma,w,i}^{11} = \sum_{\alpha \in B} \tau_{\alpha,i}^{10} \tau_{\gamma,\alpha,w}^7 \tau_{\gamma,\alpha,w}^9 \quad (3r_D r_T r_V N_o) \quad (4245)$$

$${}^2R_{i,\gamma}^2 \leftarrow - \sum_{w \in D} {}^2D_{i,w}^2 \tau_{\gamma,w,i}^{11} \quad (2r_D r_T N_o) \quad (4246)$$

Raw expression

$${}^2R_{i,\epsilon}^2 \leftarrow \sum_{\gamma \in A} \sum_{j \in O} \sum_{k \in O} \sum_{l \in O} \sum_{a \in V} \sum_{b \in V} \sum_{c \in V} \sum_{d \in V} \frac{1}{2} \quad (4247)$$

$${}^1T_{a,k} {}^1T_{b,l} Y_{a,\epsilon}^{1,*} Z_{\epsilon,\gamma}^* Y_{b,\gamma}^{3,*} Y_{j,\gamma}^{4,*} {}^2D_{a,i,b,j} {}^2T_{c,j,d,i} V_{k,d,l,c}$$

Factorized expression

$$\tau_{\gamma,\delta,w}^0 = \sum_{a \in V} {}^2D_{a,w}^3 Y_{a,\gamma}^3 Y_{a,\delta}^{3,*} \quad (3r_D r_T^2 N_v) \quad (4248)$$

$$\tau_{\gamma,\delta,w}^1 = \sum_{i \in O} {}^2D_{i,w}^4 Y_{i,\gamma}^4 Y_{i,\delta}^{4,*} \quad (3r_D r_T^2 N_o) \quad (4249)$$

$$\tau_{\gamma,\delta,w}^2 = \sum_{\epsilon \in A} Z_{\delta,\epsilon}^* \tau_{\gamma,\epsilon,w}^0 \tau_{\gamma,\epsilon,w}^1 \quad (3r_D r_T^3) \quad (4250)$$

$$\tau_{\gamma,\alpha}^3 = \sum_{a \in V} W_{a,\alpha}^4 Y_{a,\gamma}^1 \quad (2r_T r_V N_v) \quad (4251)$$

$$\tau_{\gamma,\alpha}^4 = \sum_{i \in O} W_{i,\alpha}^3 Y_{i,\gamma}^2 \quad (2r_T r_V N_o) \quad (4252)$$

$$\tau_{\gamma,\alpha}^5 = \sum_{\beta \in B} X_{\alpha,\beta} \tau_{\gamma,\beta}^3 \tau_{\gamma,\beta}^4 \quad (3r_T r_V^2) \quad (4253)$$

$$\tau_{\gamma,\alpha}^6 = \sum_{\delta \in A} Z_{\delta,\gamma} \tau_{\delta,\alpha}^5 \quad (2r_T^2 r_V) \quad (4254)$$

$$\tau_{\gamma,\alpha,w}^7 = \sum_{\delta \in A} \tau_{\delta,\alpha}^6 \tau_{\delta,\gamma,w}^2 \quad (2r_D r_T^2 r_V) \quad (4255)$$

$$\tau_{\gamma,w,i}^8 = \sum_{a \in V} {}^2D_{a,w}^1 {}^1T_{a,i} Y_{a,\gamma}^{1,*} \quad (3r_D r_T N_o N_v) \quad (4256)$$

$$\tau_{\gamma,\alpha,w}^9 = \sum_{i \in O} W_{i,\alpha}^1 \tau_{\gamma,w,i}^8 \quad (2r_D r_T r_V N_o) \quad (4257)$$

$$\tau_{\alpha,i}^{10} = \sum_{a \in V} {}^1T_{a,i} W_{a,\alpha}^2 \quad (2r_V N_o N_v) \quad (4258)$$

$$\tau_{\gamma,w,i}^{11} = \sum_{\alpha \in B} \tau_{\alpha,i}^{10} \tau_{\gamma,\alpha,w}^7 \tau_{\gamma,\alpha,w}^9 \quad (3r_D r_T r_V N_o) \quad (4259)$$

$${}^2R_{i,\gamma}^2 \leftarrow - \sum_{w \in D} {}^2D_{i,w}^2 \tau_{\gamma,w,i}^{11} \quad (2r_D r_T N_o) \quad (4260)$$

Raw expression

$${}^2R_{i,\epsilon}^2 \leftarrow \sum_{\gamma \in A} \sum_{j \in O} \sum_{k \in O} \sum_{l \in O} \sum_{a \in V} \sum_{b \in V} \sum_{c \in V} \sum_{d \in V} \frac{1}{2} \quad (4261)$$

$${}^1T_{a,k} {}^1T_{c,i} Y_{a,\epsilon}^{1,*} Z_{\epsilon,\gamma}^* Y_{b,\gamma}^{3,*} Y_{j,\gamma}^{4,*} {}^2D_{a,i,b,j} {}^2T_{b,j,d,l} V_{k,d,l,c}$$

Factorized expression

$$\tau_{\gamma,\delta,w}^0 = \sum_{a \in V} {}^2D_{a,w}^3 Y_{a,\gamma}^1 Y_{a,\delta}^{3,*} \quad (3r_D r_T^2 N_v) \quad (4262)$$

$$\tau_{\gamma,\delta,w}^1 = \sum_{i \in O} {}^2D_{i,w}^4 Y_{i,\gamma}^2 Y_{i,\delta}^{4,*} \quad (3r_D r_T^2 N_o) \quad (4263)$$

$$\tau_{\gamma,\delta,w}^2 = \sum_{\epsilon \in A} Z_{\delta,\epsilon}^* \tau_{\gamma,\epsilon,w}^0 \tau_{\gamma,\epsilon,w}^1 \quad (3r_D r_T^3) \quad (4264)$$



$$\tau^3_{\gamma,\delta,w} = \sum_{\epsilon \in A} Z_{\epsilon,\gamma} \tau^2_{\epsilon,\delta,w} \quad (2r_D r_T^3) \quad (4265)$$

$$\tau^3_{\gamma,\delta,w} = \sum_{\epsilon \in A} Z_{\gamma,\epsilon} \tau^2_{\epsilon,\delta,w} \quad (2r_D r_T^3) \quad (4278)$$

$$\tau^4_{\gamma,w,i} = \sum_{a \in V} {}^2D^1_{a,w} {}^1T_{a,i} Y^{1,*}_{a,\gamma} \quad (3r_D r_T N_o N_v) \quad (4266)$$

$$\tau^4_{\gamma,w,i} = \sum_{a \in V} {}^2D^1_{a,w} {}^1T_{a,i} Y^{1,*}_{a,\gamma} \quad (3r_D r_T N_o N_v) \quad (4279)$$

$$\tau^5_{\alpha,i} = \sum_{a \in V} {}^1T_{a,i} W^4_{a,\alpha} \quad (2r_V N_o N_v) \quad (4267)$$

$$\tau^5_{\alpha,i} = \sum_{a \in V} {}^1T_{a,i} W^4_{a,\alpha} \quad (2r_V N_o N_v) \quad (4280)$$

$$\tau^6_{\alpha} = \sum_{i \in O} W^3_{i,\alpha} \tau^5_{\alpha,i} \quad (2r_V N_o) \quad (4268)$$

$$\tau^6_{\alpha} = \sum_{i \in O} W^3_{i,\alpha} \tau^5_{\alpha,i} \quad (2r_V N_o) \quad (4281)$$

$$\tau^7_{\alpha} = \sum_{\beta \in B} \tau^6_{\beta} X_{\alpha,\beta} \quad (2r_V^2) \quad (4269)$$

$$\tau^7_{\alpha} = \sum_{\beta \in B} \tau^6_{\beta} X_{\alpha,\beta} \quad (2r_V^2) \quad (4282)$$

$$\tau^8_{i,a} = \sum_{\alpha \in B} \tau^7_{\alpha} W^1_{i,\alpha} W^2_{a,\alpha} \quad (3r_V N_o N_v) \quad (4270)$$

$$\tau^8_{i,a} = \sum_{\alpha \in B} \tau^7_{\alpha} W^1_{i,\alpha} W^2_{a,\alpha} \quad (3r_V N_o N_v) \quad (4283)$$

$$\tau^9_{\gamma,i} = \sum_{a \in V} Y^3_{a,\gamma} \tau^8_{i,a} \quad (2r_T N_o N_v) \quad (4271)$$

$$\tau^9_{\gamma,i} = \sum_{a \in V} Y^1_{a,\gamma} \tau^8_{i,a} \quad (2r_T N_o N_v) \quad (4284)$$

$$\tau^{10}_{\gamma,\delta,w} = \sum_{i \in O} \tau^9_{\gamma,i} \tau^4_{\delta,w,i} \quad (2r_D r_T^2 N_o) \quad (4272)$$

$$\tau^{10}_{\gamma,\delta,w} = \sum_{i \in O} \tau^9_{\gamma,i} \tau^4_{\delta,w,i} \quad (2r_D r_T^2 N_o) \quad (4285)$$

$${}^2R^2_{i,\gamma} \leftarrow - \sum_{\delta \in A} \sum_{w \in D} {}^2D^2_{i,w} Y^4_{i,\delta} \tau^{10}_{\delta,\gamma,w} \tau^3_{\delta,\gamma,w} \quad (4r_D r_T^2 N_o) \quad (4273)$$

$${}^2R^2_{i,\gamma} \leftarrow - \sum_{\delta \in A} \sum_{w \in D} {}^2D^2_{i,w} Y^2_{i,\delta} \tau^{10}_{\delta,\gamma,w} \tau^3_{\delta,\gamma,w} \quad (4r_D r_T^2 N_o) \quad (4286)$$

Raw expression

Raw expression

$${}^2R^2_{i,\epsilon} \leftarrow \sum_{\gamma \in A} \sum_{j \in O} \sum_{k \in O} \sum_{l \in O} \sum_{a \in V} \sum_{b \in V} \sum_{c \in V} \sum_{d \in V} \frac{1}{2} \quad (4274)$$

$$\begin{aligned} & {}^1T_{a,k} \quad {}^1T_{c,i} \quad Y^{1,*}_{a,\epsilon} \quad Z^*_{\epsilon,\gamma} \quad Y^{3,*}_{b,\gamma} \\ & Y^{4,*}_{j,\gamma} \quad {}^2D^{a,i,b,j} \quad {}^2T_{b,l,d,j} \quad V_{k,c,l,d} \end{aligned}$$

$${}^2R^2_{i,\epsilon} \leftarrow \sum_{\gamma \in A} \sum_{j \in O} \sum_{k \in O} \sum_{l \in O} \sum_{a \in V} \sum_{b \in V} \sum_{c \in V} \sum_{d \in V} \frac{1}{2} \quad (4287)$$

$$\begin{aligned} & {}^1T_{a,k} \quad {}^1T_{c,i} \quad Y^{1,*}_{a,\epsilon} \quad Z^*_{\epsilon,\gamma} \quad Y^{3,*}_{b,\gamma} \\ & Y^{4,*}_{j,\gamma} \quad {}^2D^{a,i,b,j} \quad {}^2T_{d,j,b,l} \quad V_{k,c,l,d} \end{aligned}$$

Factorized expression

Factorized expression

$$\tau^0_{\gamma,\delta,w} = \sum_{a \in V} {}^2D^3_{a,w} Y^3_{a,\gamma} Y^{3,*}_{a,\delta} \quad (3r_D r_T^2 N_v) \quad (4275)$$

$$\tau^0_{\gamma,\delta,w} = \sum_{a \in V} {}^2D^1_{a,w} Y^1_{a,\gamma} Y^{1,*}_{a,\delta} \quad (3r_D r_T^2 N_v) \quad (4288)$$

$$\tau^1_{\gamma,\delta,w} = \sum_{i \in O} {}^2D^4_{i,w} Y^4_{i,\gamma} Y^{4,*}_{i,\delta} \quad (3r_D r_T^2 N_o) \quad (4276)$$

$$\tau^1_{\alpha,i} = \sum_{a \in V} {}^1T_{a,i} W^2_{a,\alpha} \quad (2r_V N_o N_v) \quad (4289)$$

$$\tau^2_{\gamma,\delta,w} = \sum_{\epsilon \in A} Z^*_{\delta,\epsilon} \tau^0_{\gamma,\epsilon,w} \tau^1_{\gamma,\epsilon,w} \quad (3r_D r_T^3) \quad (4277)$$

$$\tau^2_{\gamma,\alpha,w} = \sum_{i \in O} {}^2D^4_{i,w} Y^{4,*}_{i,\gamma} \tau^1_{\alpha,i} \quad (3r_D r_T r_V N_o) \quad (4290)$$

$$\tau^3_{\gamma,w,i} = \sum_{a \in V} {}^2D^3_{a,w} {}^1T_{a,i} Y^{3,*}_{a,\gamma} \quad (3r_D r_T N_o N_v) \quad (4291)$$

$$\tau^3_{\gamma,w,i} = \sum_{a \in V} {}^2D^3_{a,w} {}^1T_{a,i} Y^{3,*}_{a,\gamma} \quad (3r_D r_T N_o N_v) \quad (4304)$$

$$\tau^4_{\gamma,\alpha,w} = \sum_{i \in O} W^1_{i,\alpha} \tau^3_{\gamma,w,i} \quad (2r_D r_T r_V N_o) \quad (4292)$$

$$\tau^4_{\gamma,\alpha,w} = \sum_{i \in O} W^1_{i,\alpha} \tau^3_{\gamma,w,i} \quad (2r_D r_T r_V N_o) \quad (4305)$$

$$\tau^5_{\gamma,\alpha} = \sum_{a \in V} W^4_{a,\alpha} Y^3_{a,\gamma} \quad (2r_T r_V N_v) \quad (4293)$$

$$\tau^5_{\gamma,\alpha} = \sum_{a \in V} W^4_{a,\alpha} Y^1_{a,\gamma} \quad (2r_T r_V N_v) \quad (4306)$$

$$\tau^6_{\gamma,\alpha} = \sum_{i \in O} W^3_{i,\alpha} Y^4_{i,\gamma} \quad (2r_T r_V N_o) \quad (4294)$$

$$\tau^6_{\gamma,\alpha} = \sum_{i \in O} W^3_{i,\alpha} Y^2_{i,\gamma} \quad (2r_T r_V N_o) \quad (4307)$$

$$\tau^7_{\gamma,\alpha} = \sum_{\beta \in B} X_{\alpha,\beta} \tau^5_{\gamma,\beta} \tau^6_{\gamma,\beta} \quad (3r_T r_V^2) \quad (4295)$$

$$\tau^7_{\gamma,\alpha} = \sum_{\beta \in B} X_{\alpha,\beta} \tau^5_{\gamma,\beta} \tau^6_{\gamma,\beta} \quad (3r_T r_V^2) \quad (4308)$$

$$\tau^8_{\gamma,\alpha} = \sum_{\delta \in A} Z_{\gamma,\delta} \tau^7_{\delta,\alpha} \quad (2r_T^2 r_V) \quad (4296)$$

$$\tau^8_{\gamma,\alpha} = \sum_{\delta \in A} Z_{\delta,\gamma} \tau^7_{\delta,\alpha} \quad (2r_T^2 r_V) \quad (4309)$$

$$\tau^9_{\gamma,\delta,w} = \sum_{\alpha \in B} \tau^8_{\gamma,\alpha} \tau^2_{\delta,\alpha,w} \tau^4_{\delta,\alpha,w} \quad (3r_D r_T^2 r_V) \quad (4297)$$

$$\tau^9_{\gamma,\delta,w} = \sum_{\alpha \in B} \tau^8_{\gamma,\alpha} \tau^2_{\delta,\alpha,w} \tau^4_{\delta,\alpha,w} \quad (3r_D r_T^2 r_V) \quad (4310)$$

$$\tau^{10}_{\gamma,\delta,w} = \sum_{\epsilon \in A} Z^*_{\delta,\epsilon} \tau^9_{\gamma,\epsilon,w} \quad (2r_D r_T^3) \quad (4298)$$

$$\tau^{10}_{\gamma,\delta,w} = \sum_{\epsilon \in A} Z^*_{\delta,\epsilon} \tau^9_{\gamma,\epsilon,w} \quad (2r_D r_T^3) \quad (4311)$$

$${}^2R^2_{i,\gamma} \leftarrow - \sum_{\delta \in A} \sum_{w \in D} {}^2D^2_{i,w} Y^2_{i,\delta} \tau^0_{\delta,\gamma,w} \tau^{10}_{\delta,\gamma,w} \quad (4r_D r_T^2 N_o) \quad (4299)$$

$${}^2R^2_{i,\gamma} \leftarrow - \sum_{\delta \in A} \sum_{w \in D} {}^2D^2_{i,w} Y^4_{i,\delta} \tau^0_{\delta,\gamma,w} \tau^{10}_{\delta,\gamma,w} \quad (4r_D r_T^2 N_o) \quad (4312)$$

Raw expression

$${}^2R^2_{i,\epsilon} \leftarrow \sum_{\gamma \in A} \sum_{j \in O} \sum_{k \in O} \sum_{l \in O} \sum_{a \in V} \sum_{b \in V} \sum_{c \in V} \sum_{d \in V} \frac{1}{2} \quad (4300)$$

$${}^1T_{a,k} {}^1T_{c,i} Y^{1,*}_{a,\epsilon} Z^*_{\epsilon,\gamma} Y^{3,*}_{b,\gamma} Y^{4,*}_{j,\gamma} {}^2D^{a,i,b,j}_{d,l,b,j} V_{k,d,l,c}$$

Raw expression

$${}^2R^2_{i,\epsilon} \leftarrow \sum_{\gamma \in A} \sum_{j \in O} \sum_{k \in O} \sum_{l \in O} \sum_{a \in V} \sum_{b \in V} \sum_{c \in V} \sum_{d \in V} \frac{1}{2} \quad (4313)$$

$${}^1T_{a,k} {}^1T_{c,j} Y^{1,*}_{a,\epsilon} Z^*_{\epsilon,\gamma} Y^{3,*}_{b,\gamma} Y^{4,*}_{j,\gamma} {}^2D^{a,i,b,j}_{b,l,d,i} V_{k,d,l,c}$$

Factorized expression

$$\tau^0_{\gamma,\delta,w} = \sum_{a \in V} {}^2D^1_{a,w} Y^3_{a,\gamma} Y^{1,*}_{a,\delta} \quad (3r_D r_T^2 N_v) \quad (4301)$$

$$\tau^0_{\gamma,\delta,w} = \sum_{a \in V} {}^2D^1_{a,w} Y^1_{a,\gamma} Y^{1,*}_{a,\delta} \quad (3r_D r_T^2 N_v) \quad (4314)$$

$$\tau^1_{\alpha,i} = \sum_{a \in V} {}^1T_{a,i} W^2_{a,\alpha} \quad (2r_V N_o N_v) \quad (4302)$$

$$\tau^1_{\gamma,\delta,w} = \sum_{i \in O} {}^2D^4_{i,w} Y^4_{i,\gamma} Y^{4,*}_{i,\delta} \quad (3r_D r_T^2 N_o) \quad (4315)$$

$$\tau^2_{\gamma,\alpha,w} = \sum_{i \in O} {}^2D^4_{i,w} Y^{4,*}_{i,\gamma} \tau^1_{\alpha,i} \quad (3r_D r_T r_V N_o) \quad (4303)$$

$$\tau^2_{\gamma,w,i} = \sum_{a \in V} {}^2D^3_{a,w} {}^1T_{a,i} Y^{3,*}_{a,\gamma} \quad (3r_D r_T N_o N_v) \quad (4316)$$

$$\tau^3_{\alpha,i} = \sum_{a \in V} {}^1T_{a,i} W^4_{a,\alpha} \quad (2r_V N_o N_v) \quad (4317)$$

$$\tau^3_{\alpha,i} = \sum_{a \in V} {}^1T_{a,i} W^4_{a,\alpha} \quad (2r_V N_o N_v) \quad (4330)$$

$$\tau^4_{\alpha} = \sum_{i \in O} W^3_{i,\alpha} \tau^3_{\alpha,i} \quad (2r_V N_o) \quad (4318)$$

$$\tau^4_{\alpha} = \sum_{i \in O} W^3_{i,\alpha} \tau^3_{\alpha,i} \quad (2r_V N_o) \quad (4331)$$

$$\tau^5_{\alpha} = \sum_{\beta \in B} \tau^4_{\beta} X_{\alpha,\beta} \quad (2r_V^2) \quad (4319)$$

$$\tau^5_{\alpha} = \sum_{\beta \in B} \tau^4_{\beta} X_{\alpha,\beta} \quad (2r_V^2) \quad (4332)$$

$$\tau^6_{i,a} = \sum_{\alpha \in B} \tau^5_{\alpha} W^1_{i,\alpha} W^2_{a,\alpha} \quad (3r_V N_o N_v) \quad (4320)$$

$$\tau^6_{i,a} = \sum_{\alpha \in B} \tau^5_{\alpha} W^1_{i,\alpha} W^2_{a,\alpha} \quad (3r_V N_o N_v) \quad (4333)$$

$$\tau^7_{\gamma,i} = \sum_{a \in V} Y^3_{a,\gamma} \tau^6_{i,a} \quad (2r_T N_o N_v) \quad (4321)$$

$$\tau^7_{\gamma,i} = \sum_{a \in V} Y^1_{a,\gamma} \tau^6_{i,a} \quad (2r_T N_o N_v) \quad (4334)$$

$$\tau^8_{\gamma,\delta,w} = \sum_{i \in O} \tau^7_{\gamma,i} \tau^2_{\delta,w,i} \quad (2r_D r_T^2 N_o) \quad (4322)$$

$$\tau^8_{\gamma,\delta,w} = \sum_{i \in O} \tau^7_{\gamma,i} \tau^2_{\delta,w,i} \quad (2r_D r_T^2 N_o) \quad (4335)$$

$$\tau^9_{\gamma,\delta,w} = \sum_{\epsilon \in A} Z^*_{\delta,\epsilon} \tau^1_{\gamma,\epsilon,w} \tau^8_{\gamma,\epsilon,w} \quad (3r_D r_T^3) \quad (4323)$$

$$\tau^9_{\gamma,\delta,w} = \sum_{\epsilon \in A} Z^*_{\delta,\epsilon} \tau^1_{\gamma,\epsilon,w} \tau^8_{\gamma,\epsilon,w} \quad (3r_D r_T^3) \quad (4336)$$

$$\tau^{10}_{\gamma,\delta,w} = \sum_{\epsilon \in A} Z_{\gamma,\epsilon} \tau^9_{\epsilon,\delta,w} \quad (2r_D r_T^3) \quad (4324)$$

$$\tau^{10}_{\gamma,\delta,w} = \sum_{\epsilon \in A} Z_{\epsilon,\gamma} \tau^9_{\epsilon,\delta,w} \quad (2r_D r_T^3) \quad (4337)$$

$${}^2R^2_{i,\gamma} \leftarrow - \sum_{\delta \in A} \sum_{w \in D} {}^2D^2_{i,w} Y^2_{i,\delta} \tau^0_{\delta,\gamma,w} \tau^{10}_{\delta,\gamma,w} \quad (4r_D r_T^2 N_o) \quad (4325)$$

$${}^2R^2_{i,\gamma} \leftarrow - \sum_{\delta \in A} \sum_{w \in D} {}^2D^2_{i,w} Y^4_{i,\delta} \tau^0_{\delta,\gamma,w} \tau^{10}_{\delta,\gamma,w} \quad (4r_D r_T^2 N_o) \quad (4338)$$

Raw expression

$${}^2R^2_{i,\epsilon} \leftarrow \sum_{\gamma \in A} \sum_{j \in O} \sum_{k \in O} \sum_{l \in O} \sum_{a \in V} \sum_{b \in V} \sum_{c \in V} \sum_{d \in V} \frac{1}{2} \quad (4326)$$

$$\begin{aligned} & {}^1T_{a,k} \quad {}^1T_{c,j} \quad Y^{1,*}_{a,\epsilon} \quad Z^*_{\epsilon,\gamma} \quad Y^{3,*}_{b,\gamma} \\ & Y^{4,*}_{j,\gamma} \quad {}^2D^{a,i,b,j} \quad {}^2T_{d,i,b,l} \quad V_{k,d,l,c} \end{aligned}$$

Factorized expression

$$\tau^0_{\gamma,\delta,w} = \sum_{a \in V} {}^2D^1_{a,w} Y^3_{a,\gamma} Y^{1,*}_{a,\delta} \quad (3r_D r_T^2 N_v) \quad (4327)$$

$$\tau^1_{\gamma,\delta,w} = \sum_{i \in O} {}^2D^4_{i,w} Y^2_{i,\gamma} Y^{4,*}_{i,\delta} \quad (3r_D r_T^2 N_o) \quad (4328)$$

$$\tau^2_{\gamma,w,i} = \sum_{a \in V} {}^2D^3_{a,w} {}^1T_{a,i} Y^{3,*}_{a,\gamma} \quad (3r_D r_T N_o N_v) \quad (4329)$$

Raw expression

$${}^2R^2_{i,\epsilon} \leftarrow \sum_{\gamma \in A} \sum_{j \in O} \sum_{k \in O} \sum_{l \in O} \sum_{a \in V} \sum_{b \in V} \sum_{c \in V} \sum_{d \in V} \frac{1}{2} \quad (4339)$$

$$\begin{aligned} & {}^1T_{a,k} \quad {}^1T_{c,l} \quad Y^{1,*}_{a,\epsilon} \quad Z^*_{\epsilon,\gamma} \quad Y^{3,*}_{b,\gamma} \\ & Y^{4,*}_{j,\gamma} \quad {}^2D^{a,i,b,j} \quad {}^2T_{b,j,d,i} \quad V_{k,c,l,d} \end{aligned}$$

Factorized expression

$$\tau^0_{\gamma,\delta,w} = \sum_{a \in V} {}^2D^1_{a,w} Y^1_{a,\gamma} Y^{1,*}_{a,\delta} \quad (3r_D r_T^2 N_v) \quad (4340)$$

$$\tau^1_{\gamma,\delta,w} = \sum_{a \in V} {}^2D^3_{a,w} Y^3_{a,\gamma} Y^{3,*}_{a,\delta} \quad (3r_D r_T^2 N_v) \quad (4341)$$

$$\tau^2_{\gamma,\delta,w} = \sum_{i \in O} {}^2D^4_{i,w} Y^4_{i,\gamma} Y^{4,*}_{i,\delta} \quad (3r_D r_T^2 N_o) \quad (4342)$$

$$\tau^3_{\gamma,\delta,w} = \sum_{\epsilon \in A} Z^*_{\delta,\epsilon} \tau^1_{\gamma,\epsilon,w} \tau^2_{\gamma,\epsilon,w} \quad (3r_D r_T^3) \quad (4343)$$

$$\tau^3_{\gamma,\delta,w} = \sum_{\epsilon \in A} Z_{\epsilon,\gamma} \tau^2_{\epsilon,\delta,w} \quad (2r_D r_T^3) \quad (4356)$$

$$\tau^4_{\gamma,\delta,w} = \sum_{\epsilon \in A} Z_{\gamma,\epsilon} \tau^3_{\epsilon,\delta,w} \quad (2r_D r_T^3) \quad (4344)$$

$$\tau^4_{\gamma,\delta,w} = \sum_{a \in V} {}^2D^1_{a,w} Y^3_{a,\gamma} Y^{1,*}_{a,\delta} \quad (3r_D r_T^2 N_v) \quad (4357)$$

$$\tau^5_{\alpha,i} = \sum_{a \in V} {}^1T_{a,i} W^2_{a,\alpha} \quad (2r_V N_o N_v) \quad (4345)$$

$$\tau^5_{\alpha,i} = \sum_{a \in V} {}^1T_{a,i} W^2_{a,\alpha} \quad (2r_V N_o N_v) \quad (4358)$$

$$\tau^6_{\alpha} = \sum_{i \in O} W^1_{i,\alpha} \tau^5_{\alpha,i} \quad (2r_V N_o) \quad (4346)$$

$$\tau^6_{\alpha} = \sum_{i \in O} W^1_{i,\alpha} \tau^5_{\alpha,i} \quad (2r_V N_o) \quad (4359)$$

$$\tau^7_{\alpha} = \sum_{\beta \in B} \tau^6_{\beta} X_{\beta,\alpha} \quad (2r_V^2) \quad (4347)$$

$$\tau^7_{\alpha} = \sum_{\beta \in B} \tau^6_{\beta} X_{\beta,\alpha} \quad (2r_V^2) \quad (4360)$$

$$\tau^8_{i,a} = \sum_{\alpha \in B} \tau^7_{\alpha} W^3_{i,\alpha} W^4_{a,\alpha} \quad (3r_V N_o N_v) \quad (4348)$$

$$\tau^8_{i,a} = \sum_{\alpha \in B} \tau^7_{\alpha} W^3_{i,\alpha} W^4_{a,\alpha} \quad (3r_V N_o N_v) \quad (4361)$$

$$\tau^9_{i,j} = \sum_{a \in V} {}^1T_{a,i} \tau^8_{j,a} \quad (2N_o^2 N_v) \quad (4349)$$

$$\tau^9_{i,j} = \sum_{a \in V} {}^1T_{a,i} \tau^8_{j,a} \quad (2N_o^2 N_v) \quad (4362)$$

$$\tau^{10}_{\gamma,i} = \sum_{j \in O} Y^2_{j,\gamma} \tau^9_{i,j} \quad (2r_T N_o^2) \quad (4350)$$

$$\tau^{10}_{\gamma,i} = \sum_{j \in O} Y^4_{j,\gamma} \tau^9_{i,j} \quad (2r_T N_o^2) \quad (4363)$$

$${}^2R^2_{i,\gamma} \leftarrow - \sum_{\delta \in A} \sum_{w \in D} {}^2D^2_{i,w} \tau^{10}_{\delta,i} \tau^0_{\delta,\gamma,w} \tau^4_{\delta,\gamma,w} \quad (4r_D r_T^2 N_o) \quad (4351)$$

$${}^2R^2_{i,\gamma} \leftarrow - \sum_{\delta \in A} \sum_{w \in D} {}^2D^2_{i,w} \tau^{10}_{\delta,i} \tau^3_{\delta,\gamma,w} \tau^4_{\delta,\gamma,w} \quad (4r_D r_T^2 N_o) \quad (4364)$$

Raw expression

Raw expression

$${}^2R^2_{i,\epsilon} \leftarrow \sum_{\gamma \in A} \sum_{j \in O} \sum_{k \in O} \sum_{l \in O} \sum_{a \in V} \sum_{b \in V} \sum_{c \in V} \sum_{d \in V} \frac{1}{2} \quad (4352)$$

$${}^1T_{a,k} {}^1T_{c,l} Y^{1,*}_{a,\epsilon} Z^*_{\epsilon,\gamma} Y^{3,*}_{b,\gamma} Y^{4,*}_{j,\gamma} {}^2D^{a,i,b,j} {}^2T_{d,i,b,j} V_{k,c,l,d}$$

$${}^2R^2_{i,\epsilon} \leftarrow \sum_{\gamma \in A} \sum_{j \in O} \sum_{k \in O} \sum_{l \in O} \sum_{a \in V} \sum_{b \in V} \sum_{c \in V} \sum_{d \in V} \frac{1}{2} \quad (4365)$$

$${}^1T_{b,k} {}^1T_{c,i} Y^{1,*}_{a,\epsilon} Z^*_{\epsilon,\gamma} Y^{3,*}_{b,\gamma} Y^{4,*}_{j,\gamma} {}^2D^{a,i,b,j} {}^2T_{a,l,d,j} V_{k,d,l,c}$$

Factorized expression

Factorized expression

$$\tau^0_{\gamma,\delta,w} = \sum_{a \in V} {}^2D^3_{a,w} Y^1_{a,\gamma} Y^{3,*}_{a,\delta} \quad (3r_D r_T^2 N_v) \quad (4353)$$

$$\tau^0_{\gamma,\delta,w} = \sum_{a \in V} {}^2D^1_{a,w} Y^1_{a,\gamma} Y^{1,*}_{a,\delta} \quad (3r_D r_T^2 N_v) \quad (4366)$$

$$\tau^1_{\gamma,\delta,w} = \sum_{i \in O} {}^2D^4_{i,w} Y^2_{i,\gamma} Y^{4,*}_{i,\delta} \quad (3r_D r_T^2 N_o) \quad (4354)$$

$$\tau^1_{\gamma,\delta,w} = \sum_{a \in V} {}^2D^3_{a,w} Y^3_{a,\gamma} Y^{3,*}_{a,\delta} \quad (3r_D r_T^2 N_v) \quad (4367)$$

$$\tau^2_{\gamma,\delta,w} = \sum_{\epsilon \in A} Z^*_{\delta,\epsilon} \tau^0_{\gamma,\epsilon,w} \tau^1_{\gamma,\epsilon,w} \quad (3r_D r_T^3) \quad (4355)$$

$$\tau^2_{\alpha,i} = \sum_{a \in V} {}^1T_{a,i} W^2_{a,\alpha} \quad (2r_V N_o N_v) \quad (4368)$$

$$\tau^3_{\alpha} = \sum_{i \in O} W^1_{i,\alpha} \tau^2_{\alpha,i} \quad (2r_V N_o) \quad (4369)$$

$$\tau^3_{\alpha} = \sum_{i \in O} W^1_{i,\alpha} \tau^2_{\alpha,i} \quad (2r_V N_o) \quad (4382)$$

$$\tau^4_{\alpha} = \sum_{\beta \in B} \tau^3_{\beta} X_{\beta,\alpha} \quad (2r_V^2) \quad (4370)$$

$$\tau^4_{\alpha} = \sum_{\beta \in B} \tau^3_{\beta} X_{\beta,\alpha} \quad (2r_V^2) \quad (4383)$$

$$\tau^5_{i,a} = \sum_{\alpha \in B} \tau^4_{\alpha} W^3_{i,\alpha} W^4_{a,\alpha} \quad (3r_V N_o N_v) \quad (4371)$$

$$\tau^5_{i,a} = \sum_{\alpha \in B} \tau^4_{\alpha} W^3_{i,\alpha} W^4_{a,\alpha} \quad (3r_V N_o N_v) \quad (4384)$$

$$\tau^6_{i,j} = \sum_{a \in V} {}^1T_{a,i} \tau^5_{j,a} \quad (2N_o^2 N_v) \quad (4372)$$

$$\tau^6_{i,j} = \sum_{a \in V} {}^1T_{a,i} \tau^5_{j,a} \quad (2N_o^2 N_v) \quad (4385)$$

$$\tau^7_{\gamma,i} = \sum_{j \in O} Y^4_{j,\gamma} \tau^6_{i,j} \quad (2r_T N_o^2) \quad (4373)$$

$$\tau^7_{\gamma,i} = \sum_{j \in O} Y^2_{j,\gamma} \tau^6_{i,j} \quad (2r_T N_o^2) \quad (4386)$$

$$\tau^8_{\gamma,\delta,w} = \sum_{i \in O} {}^2D^4_{i,w} Y^{4,*}_{i,\delta} \tau^7_{\gamma,i} \quad (3r_D r_T^2 N_o) \quad (4374)$$

$$\tau^8_{\gamma,\delta,w} = \sum_{i \in O} {}^2D^4_{i,w} Y^{4,*}_{i,\delta} \tau^7_{\gamma,i} \quad (3r_D r_T^2 N_o) \quad (4387)$$

$$\tau^9_{\gamma,\delta,w} = \sum_{\epsilon \in A} Z^*_{\delta,\epsilon} \tau^1_{\gamma,\epsilon,w} \tau^8_{\gamma,\epsilon,w} \quad (3r_D r_T^3) \quad (4375)$$

$$\tau^9_{\gamma,\delta,w} = \sum_{\epsilon \in A} Z^*_{\delta,\epsilon} \tau^1_{\gamma,\epsilon,w} \tau^8_{\gamma,\epsilon,w} \quad (3r_D r_T^3) \quad (4388)$$

$$\tau^{10}_{\gamma,\delta,w} = \sum_{\epsilon \in A} Z_{\gamma,\epsilon} \tau^9_{\epsilon,\delta,w} \quad (2r_D r_T^3) \quad (4376)$$

$$\tau^{10}_{\gamma,\delta,w} = \sum_{\epsilon \in A} Z_{\epsilon,\gamma} \tau^9_{\epsilon,\delta,w} \quad (2r_D r_T^3) \quad (4389)$$

$${}^2R^2_{i,\gamma} \leftarrow - \sum_{\delta \in A} \sum_{w \in D} {}^2D^2_{i,w} Y^2_{i,\delta} \tau^0_{\delta,\gamma,w} \tau^{10}_{\delta,\gamma,w} \quad (4r_D r_T^2 N_o) \quad (4377)$$

$${}^2R^2_{i,\gamma} \leftarrow - \sum_{\delta \in A} \sum_{w \in D} {}^2D^2_{i,w} Y^4_{i,\delta} \tau^0_{\delta,\gamma,w} \tau^{10}_{\delta,\gamma,w} \quad (4r_D r_T^2 N_o) \quad (4390)$$

Raw expression

$${}^2R^2_{i,\epsilon} \leftarrow \sum_{\gamma \in A} \sum_{j \in O} \sum_{k \in O} \sum_{l \in O} \sum_{a \in V} \sum_{b \in V} \sum_{c \in V} \sum_{d \in V} \frac{1}{2} \quad (4378)$$

$${}^1T_{b,k} \quad {}^1T_{c,i} \quad Y^{1,*}_{a,\epsilon} \quad Z^*_{\epsilon,\gamma} \quad Y^{3,*}_{b,\gamma} \quad Y^{4,*}_{j,\gamma} \quad {}^2D^{a,i,b,j} \quad {}^2T_{d,j,a,l} \quad V_{k,d,l,c}$$

Raw expression

$${}^2R^2_{i,\epsilon} \leftarrow \sum_{\gamma \in A} \sum_{j \in O} \sum_{k \in O} \sum_{l \in O} \sum_{a \in V} \sum_{b \in V} \sum_{c \in V} \sum_{d \in V} \frac{1}{2} \quad (4391)$$

$${}^1T_{b,k} \quad {}^1T_{c,j} \quad Y^{1,*}_{a,\epsilon} \quad Z^*_{\epsilon,\gamma} \quad Y^{3,*}_{b,\gamma} \quad Y^{4,*}_{j,\gamma} \quad {}^2D^{a,i,b,j} \quad {}^2T_{a,i,d,l} \quad V_{k,d,l,c}$$

Factorized expression

$$\tau^0_{\gamma,\delta,w} = \sum_{a \in V} {}^2D^1_{a,w} Y^3_{a,\gamma} Y^{1,*}_{a,\delta} \quad (3r_D r_T^2 N_v) \quad (4379)$$

$$\tau^0_{\gamma,w,i} = \sum_{a \in V} {}^2D^3_{a,w} {}^1T_{a,i} Y^{3,*}_{a,\gamma} \quad (3r_D r_T N_o N_v) \quad (4392)$$

$$\tau^1_{\gamma,\delta,w} = \sum_{a \in V} {}^2D^3_{a,w} Y^1_{a,\gamma} Y^{3,*}_{a,\delta} \quad (3r_D r_T^2 N_v) \quad (4380)$$

$$\tau^1_{\gamma,\alpha} = \sum_{a \in V} W^2_{a,\alpha} Y^1_{a,\gamma} \quad (2r_T r_V N_v) \quad (4393)$$

$$\tau^2_{\alpha,i} = \sum_{a \in V} {}^1T_{a,i} W^2_{a,\alpha} \quad (2r_V N_o N_v) \quad (4381)$$

$$\tau^2_{\gamma,\alpha,i} = \sum_{\beta \in B} W^1_{i,\beta} X_{\beta,\alpha} \tau^1_{\gamma,\beta} \quad (3r_T r_V^2 N_o) \quad (4394)$$

$$\tau^3_{\gamma,\alpha} = \sum_{a \in V} W^4_{a,\alpha} Y^3_{a,\gamma} \quad (2r_T r_V N_v) \quad (4395)$$

$$\tau^2_{\gamma,\alpha,i} = \sum_{\beta \in B} X_{\alpha,\beta} W^3_{i,\beta} \tau^1_{\gamma,\beta} \quad (3r_T r_V^2 N_o) \quad (4407)$$

$$\tau^4_{\gamma,\alpha,i} = \sum_{\delta \in A} Z_{\gamma,\delta} Y^4_{i,\delta} \tau^3_{\delta,\alpha} \quad (3r_T^2 r_V N_o) \quad (4396)$$

$$\tau^3_{\gamma,\alpha} = \sum_{a \in V} W^2_{a,\alpha} Y^3_{a,\gamma} \quad (2r_T r_V N_v) \quad (4408)$$

$$\tau^5_{\gamma,i,j,k} = \sum_{\alpha \in B} W^3_{j,\alpha} \tau^2_{\gamma,\alpha,i} \tau^4_{\gamma,\alpha,k} \quad (3r_T r_V N_o^3) \quad (4397)$$

$$\tau^4_{\gamma,\alpha,i} = \sum_{\delta \in A} Z_{\gamma,\delta} Y^4_{i,\delta} \tau^3_{\delta,\alpha} \quad (3r_T^2 r_V N_o) \quad (4409)$$

$$\tau^6_{i,j,k,l} = \sum_{\gamma \in A} Y^2_{k,\gamma} \tau^5_{\gamma,i,j,l} \quad (2r_T N_o^4) \quad (4398)$$

$$\tau^5_{\gamma,i,j,k} = \sum_{\alpha \in B} W^1_{i,\alpha} \tau^2_{\gamma,\alpha,j} \tau^4_{\gamma,\alpha,k} \quad (3r_T r_V N_o^3) \quad (4410)$$

$$\tau^7_{\gamma,w,i,j} = \sum_{k \in O} \sum_{l \in O} {}^2D^4_{k,w} Y^{4,*}_{k,\gamma} \tau^0_{\gamma,w,l} \tau^6_{i,l,j,k} \quad (4r_D r_T N_o^4) \quad (4399)$$

$$\tau^6_{i,j,k,l} = \sum_{\gamma \in A} Y^2_{k,\gamma} \tau^5_{\gamma,i,j,l} \quad (2r_T N_o^4) \quad (4411)$$

$$\tau^8_{\gamma,w,i,j} = \sum_{\delta \in A} Z^*_{\gamma,\delta} \tau^7_{\delta,w,i,j} \quad (2r_D r_T^2 N_o^2) \quad (4400)$$

$$\tau^7_{\gamma,w,i,j} = \sum_{k \in O} \sum_{l \in O} {}^2D^4_{k,w} Y^{4,*}_{k,\gamma} \tau^0_{\gamma,w,l} \tau^6_{i,l,k,j} \quad (4r_D r_T N_o^4) \quad (4412)$$

$$\tau^9_{\gamma,w,i} = \sum_{a \in V} {}^2D^1_{a,w} {}^1T_{a,i} Y^{1,*}_{a,\gamma} \quad (3r_D r_T N_o N_v) \quad (4401)$$

$$\tau^8_{\gamma,w,i,j} = \sum_{\delta \in A} Z^*_{\gamma,\delta} \tau^7_{\delta,w,i,j} \quad (2r_D r_T^2 N_o^2) \quad (4413)$$

$$\tau^{10}_{\gamma,w,i} = \sum_{j \in O} \tau^9_{\gamma,w,j} \tau^8_{\gamma,w,j,i} \quad (2r_D r_T N_o^2) \quad (4402)$$

$$\tau^9_{\gamma,w,i} = \sum_{a \in V} {}^2D^1_{a,w} {}^1T_{a,i} Y^{1,*}_{a,\gamma} \quad (3r_D r_T N_o N_v) \quad (4414)$$

$${}^2R^2_{i,\gamma} \leftarrow \sum_{w \in D} \frac{1}{2} {}^2D^2_{i,w} \tau^{10}_{\gamma,w,i} \quad (2r_D r_T N_o) \quad (4403)$$

$$\tau^{10}_{\gamma,w,i} = \sum_{j \in O} \tau^9_{\gamma,w,j} \tau^8_{\gamma,w,j,i} \quad (2r_D r_T N_o^2) \quad (4415)$$

Raw expression

$${}^2R^2_{i,\epsilon} \leftarrow \sum_{\gamma \in A} \sum_{j \in O} \sum_{k \in O} \sum_{l \in O} \sum_{a \in V} \sum_{b \in V} \sum_{c \in V} \sum_{d \in V} \frac{1}{2} \quad (4404)$$

$${}^1T_{b,k} {}^1T_{c,j} Y^{1,*}_{a,\epsilon} Z^*_{\epsilon,\gamma} Y^{3,*}_{b,\gamma} Y^{4,*}_{j,\gamma} {}^2D^{a,i,b,j} {}^2T_{a,l,d,i} V_{k,c,l,d}$$

Factorized expression

$$\tau^0_{\gamma,w,i} = \sum_{a \in V} {}^2D^3_{a,w} {}^1T_{a,i} Y^{3,*}_{a,\gamma} \quad (3r_D r_T N_o N_v) \quad (4405)$$

$$\tau^1_{\gamma,\alpha} = \sum_{a \in V} W^4_{a,\alpha} Y^1_{a,\gamma} \quad (2r_T r_V N_v) \quad (4406)$$

$${}^2R^2_{i,\gamma} \leftarrow \sum_{w \in D} \frac{1}{2} {}^2D^2_{i,w} \tau^{10}_{\gamma,w,i} \quad (2r_D r_T N_o) \quad (4416)$$

Raw expression

$${}^2R^2_{i,\epsilon} \leftarrow \sum_{\gamma \in A} \sum_{j \in O} \sum_{k \in O} \sum_{l \in O} \sum_{a \in V} \sum_{b \in V} \sum_{c \in V} \sum_{d \in V} \frac{1}{2} \quad (4417)$$

$${}^1T_{b,k} {}^1T_{c,j} Y^{1,*}_{a,\epsilon} Z^*_{\epsilon,\gamma} Y^{3,*}_{b,\gamma} Y^{4,*}_{j,\gamma} {}^2D^{a,i,b,j} {}^2T_{d,i,a,l} V_{k,c,l,d}$$

Factorized expression

$$\tau^0_{\gamma,\delta,w} = \sum_{a \in V} {}^2D^3_{a,w} Y^1_{a,\gamma} Y^{3,*}_{a,\delta} \quad (3r_D r_T^2 N_v) \quad (4418)$$

$$\tau^1_{\gamma,\alpha} = \sum_{i \in O} W^3_{i,\alpha} Y^2_{i,\gamma} \quad (2r_T r_V N_o) \quad (4419)$$

$$\tau^1_{\gamma,\alpha} = \sum_{a \in V} W^4_{a,\alpha} Y^1_{a,\gamma} \quad (2r_T r_V N_v) \quad (4432)$$

$$\tau^2_{\gamma,\alpha} = \sum_{a \in V} W^4_{a,\alpha} Y^3_{a,\gamma} \quad (2r_T r_V N_v) \quad (4420)$$

$$\tau^2_{\gamma,\alpha,i} = \sum_{\delta \in A} Y^2_{i,\delta} Z_{\delta,\gamma} \tau^1_{\delta,\alpha} \quad (3r_T^2 r_V N_o) \quad (4433)$$

$$\tau^3_{\gamma,\alpha,i} = \sum_{\delta \in A} Z_{\gamma,\delta} Y^4_{i,\delta} \tau^2_{\delta,\alpha} \quad (3r_T^2 r_V N_o) \quad (4421)$$

$$\tau^3_{\gamma,\alpha} = \sum_{i \in O} W^3_{i,\alpha} Y^4_{i,\gamma} \quad (2r_T r_V N_o) \quad (4434)$$

$$\tau^4_{\gamma,\alpha,w} = \sum_{\delta \in A} \sum_{i \in O} {}^2D^4_{i,w} Y^{4,*}_{i,\gamma} \tau^1_{\delta,\alpha} \tau^0_{\delta,\gamma,w} \tau^3_{\delta,\alpha,i} \quad (5r_D r_T^2 r_V N_o) \quad (4422)$$

$$\tau^4_{\gamma,\alpha,w} = \sum_{\delta \in A} \sum_{i \in O} {}^2D^4_{i,w} Y^{4,*}_{i,\gamma} \tau^3_{\delta,\alpha} \tau^0_{\delta,\gamma,w} \tau^2_{\delta,\alpha,i} \quad (5r_D r_T^2 r_V N_o) \quad (4435)$$

$$\tau^5_{\gamma,\alpha,w} = \sum_{\beta \in B} X_{\alpha,\beta} \tau^4_{\gamma,\beta,w} \quad (2r_D r_T r_V^2) \quad (4423)$$

$$\tau^5_{\gamma,\alpha,w} = \sum_{\beta \in B} X_{\alpha,\beta} \tau^4_{\gamma,\beta,w} \quad (2r_D r_T r_V^2) \quad (4436)$$

$$\tau^6_{\gamma,\alpha,w} = \sum_{\delta \in A} Z^*_{\gamma,\delta} \tau^5_{\delta,\alpha,w} \quad (2r_D r_T^2 r_V) \quad (4424)$$

$$\tau^6_{\gamma,\alpha,w} = \sum_{\delta \in A} Z^*_{\gamma,\delta} \tau^5_{\delta,\alpha,w} \quad (2r_D r_T^2 r_V) \quad (4437)$$

$$\tau^7_{\gamma,w,i} = \sum_{a \in V} {}^2D^1_{a,w} {}^1T_{a,i} Y^{1,*}_{a,\gamma} \quad (3r_D r_T N_o N_v) \quad (4425)$$

$$\tau^7_{\gamma,w,i} = \sum_{a \in V} {}^2D^1_{a,w} {}^1T_{a,i} Y^{1,*}_{a,\gamma} \quad (3r_D r_T N_o N_v) \quad (4438)$$

$$\tau^8_{\gamma,\alpha,w} = \sum_{i \in O} W^1_{i,\alpha} \tau^7_{\gamma,w,i} \quad (2r_D r_T r_V N_o) \quad (4426)$$

$$\tau^8_{\gamma,\alpha,w} = \sum_{i \in O} W^1_{i,\alpha} \tau^7_{\gamma,w,i} \quad (2r_D r_T r_V N_o) \quad (4439)$$

$$\tau^9_{\alpha,i} = \sum_{a \in V} {}^1T_{a,i} W^2_{a,\alpha} \quad (2r_V N_o N_v) \quad (4427)$$

$$\tau^9_{\alpha,i} = \sum_{a \in V} {}^1T_{a,i} W^2_{a,\alpha} \quad (2r_V N_o N_v) \quad (4440)$$

$$\tau^{10}_{\gamma,w,i} = \sum_{\alpha \in B} \tau^9_{\alpha,i} \tau^6_{\gamma,\alpha,w} \tau^8_{\gamma,\alpha,w} \quad (3r_D r_T r_V N_o) \quad (4428)$$

$$\tau^{10}_{\gamma,w,i} = \sum_{\alpha \in B} \tau^9_{\alpha,i} \tau^6_{\gamma,\alpha,w} \tau^8_{\gamma,\alpha,w} \quad (3r_D r_T r_V N_o) \quad (4441)$$

$${}^2R^2_{i,\gamma} \leftarrow \sum_{w \in D} \frac{1}{2} {}^2D^2_{i,w} \tau^{10}_{\gamma,w,i} \quad (2r_D r_T N_o) \quad (4429)$$

$${}^2R^2_{i,\gamma} \leftarrow \sum_{w \in D} \frac{1}{2} {}^2D^2_{i,w} \tau^{10}_{\gamma,w,i} \quad (2r_D r_T N_o) \quad (4442)$$

Raw expression

Raw expression

$${}^2R^2_{i,\epsilon} \leftarrow \sum_{\gamma \in A} \sum_{j \in O} \sum_{k \in O} \sum_{l \in O} \sum_{a \in V} \sum_{b \in V} \sum_{c \in V} \sum_{d \in V} \frac{1}{2} \quad (4430)$$

$${}^1T_{b,k} {}^1T_{c,j} Y^{1,*}_{a,\epsilon} Z^*_{\epsilon,\gamma} Y^{3,*}_{b,\gamma} Y^{4,*}_{j,\gamma} {}^2D^{a,i,b,j} {}^2T_{d,l,a,i} V_{k,d,l,c}$$

$${}^2R^2_{i,\epsilon} \leftarrow \sum_{\gamma \in A} \sum_{j \in O} \sum_{k \in O} \sum_{l \in O} \sum_{a \in V} \sum_{b \in V} \sum_{c \in V} \sum_{d \in V} \frac{1}{2} \quad (4443)$$

$${}^1T_{b,k} {}^1T_{c,l} Y^{1,*}_{a,\epsilon} Z^*_{\epsilon,\gamma} Y^{3,*}_{b,\gamma} Y^{4,*}_{j,\gamma} {}^2D^{a,i,b,j} {}^2T_{a,i,d,j} V_{k,c,l,d}$$

Factorized expression

Factorized expression

$$\tau^0_{\gamma,\delta,w} = \sum_{a \in V} {}^2D^3_{a,w} Y^3_{a,\gamma} Y^{3,*}_{a,\delta} \quad (3r_D r_T^2 N_v) \quad (4431)$$

$$\tau^0_{\gamma,\alpha} = \sum_{a \in V} W^2_{a,\alpha} Y^3_{a,\gamma} \quad (2r_T r_V N_v) \quad (4444)$$

$$\tau^1_{\alpha,i} = \sum_{a \in V} {}^1T_{a,i} W^4_{a,\alpha} \quad (2r_V N_o N_v) \quad (4445)$$

$$\tau^2_{\alpha,i,j} = \sum_{\beta \in B} X_{\alpha,\beta} W^3_{j,\beta} \tau^1_{\beta,i} \quad (3r_V^2 N_o^2) \quad (4446)$$

$$\tau^3_{\gamma,\alpha,i} = \sum_{j \in O} Y^4_{j,\gamma} \tau^2_{\alpha,i,j} \quad (2r_T r_V N_o^2) \quad (4447)$$

$$\tau^4_{\gamma,i,j} = \sum_{\alpha \in B} W^1_{j,\alpha} \tau^0_{\gamma,\alpha} \tau^3_{\gamma,\alpha,i} \quad (3r_T r_V N_o^2) \quad (4448)$$

$$\tau^5_{\gamma,i,j} = \sum_{\delta \in A} Z_{\gamma,\delta} \tau^4_{\delta,i,j} \quad (2r_T^2 N_o^2) \quad (4449)$$

$$\tau^6_{\gamma,\delta,w} = \sum_{a \in V} {}^2D^3_{a,w} Y^1_{a,\gamma} Y^{3,*}_{a,\delta} \quad (3r_D r_T^2 N_v) \quad (4450)$$

$$\tau^7_{\gamma,\delta,w} = \sum_{i \in O} {}^2D^4_{i,w} Y^2_{i,\gamma} Y^{4,*}_{i,\delta} \quad (3r_D r_T^2 N_o) \quad (4451)$$

$$\tau^8_{\gamma,\delta,w} = \sum_{\epsilon \in A} Z^*_{\delta,\epsilon} \tau^6_{\gamma,\epsilon,w} \tau^7_{\gamma,\epsilon,w} \quad (3r_D r_T^3) \quad (4452)$$

$$\tau^9_{\gamma,w,i,j} = \sum_{\delta \in A} \tau^5_{\delta,i,j} \tau^8_{\delta,\gamma,w} \quad (2r_D r_T^2 N_o^2) \quad (4453)$$

$$\tau^{10}_{\gamma,w,i} = \sum_{a \in V} {}^2D^1_{a,w} {}^1T_{a,i} Y^{1,*}_{a,\gamma} \quad (3r_D r_T N_o N_v) \quad (4454)$$

$$\tau^{11}_{\gamma,w,i} = \sum_{j \in O} \tau^{10}_{\gamma,w,j} \tau^9_{\gamma,w,i,j} \quad (2r_D r_T N_o^2) \quad (4455)$$

$${}^2R^2_{i,\gamma} \leftarrow \sum_{w \in D} \frac{1}{2} {}^2D^2_{i,w} \tau^{11}_{\gamma,w,i} \quad (2r_D r_T N_o) \quad (4456)$$

Raw expression

$${}^2R^2_{i,\epsilon} \leftarrow \sum_{\gamma \in A} \sum_{j \in O} \sum_{k \in O} \sum_{l \in O} \sum_{a \in V} \sum_{b \in V} \sum_{c \in V} \sum_{d \in V} \frac{1}{2} \quad (4457)$$

$$\begin{aligned} & {}^1T_{b,k} \quad {}^1T_{c,l} \quad Y^{1,*}_{a,\epsilon} \quad Z^*_{\epsilon,\gamma} \quad Y^{3,*}_{b,\gamma} \\ & Y^{4,*}_{j,\gamma} \quad {}^2D^{a,i,b,j} \quad {}^2T_{d,j,a,i} \quad V_{k,c,l,d} \end{aligned}$$

Factorized expression

$$\tau^0_{\gamma,\alpha} = \sum_{a \in V} W^2_{a,\alpha} Y^1_{a,\gamma} \quad (2r_T r_V N_v) \quad (4458)$$

$$\tau^1_{\alpha,i} = \sum_{a \in V} {}^1T_{a,i} W^4_{a,\alpha} \quad (2r_V N_o N_v) \quad (4459)$$

$$\tau^2_{\alpha,i,j} = \sum_{\beta \in B} X_{\alpha,\beta} W^3_{j,\beta} \tau^1_{\beta,i} \quad (3r_V^2 N_o^2) \quad (4460)$$

$$\tau^3_{\gamma,\alpha,i} = \sum_{j \in O} Y^2_{j,\gamma} \tau^2_{\alpha,i,j} \quad (2r_T r_V N_o^2) \quad (4461)$$

$$\tau^4_{\gamma,i,j} = \sum_{\alpha \in B} W^1_{j,\alpha} \tau^0_{\gamma,\alpha} \tau^3_{\gamma,\alpha,i} \quad (3r_T r_V N_o^2) \quad (4462)$$

$$\tau^5_{\gamma,i,j} = \sum_{\delta \in A} Z_{\delta,\gamma} \tau^4_{\delta,i,j} \quad (2r_T^2 N_o^2) \quad (4463)$$

$$\tau^6_{\gamma,\delta,w} = \sum_{a \in V} {}^2D^3_{a,w} Y^3_{a,\gamma} Y^{3,*}_{a,\delta} \quad (3r_D r_T^2 N_v) \quad (4464)$$

$$\tau^7_{\gamma,\delta,w} = \sum_{i \in O} {}^2D^4_{i,w} Y^4_{i,\gamma} Y^{4,*}_{i,\delta} \quad (3r_D r_T^2 N_o) \quad (4465)$$

$$\tau^8_{\gamma,\delta,w} = \sum_{\epsilon \in A} Z^*_{\delta,\epsilon} \tau^6_{\gamma,\epsilon,w} \tau^7_{\gamma,\epsilon,w} \quad (3r_D r_T^3) \quad (4466)$$

$$\tau^9_{\gamma,w,i,j} = \sum_{\delta \in A} \tau^5_{\delta,i,j} \tau^8_{\delta,\gamma,w} \quad (2r_D r_T^2 N_o^2) \quad (4467)$$

$$\tau^{10}_{\gamma,w,i} = \sum_{a \in V} {}^2D^1_{a,w} {}^1T_{a,i} Y^{1,*}_{a,\gamma} \quad (3r_D r_T N_o N_v) \quad (4468)$$

$$\tau^{11}_{\gamma,w,i} = \sum_{j \in O} \tau^{10}_{\gamma,w,j} \tau^9_{\gamma,w,i,j} \quad (2r_D r_T N_o^2) \quad (4469)$$

$${}^2R^2_{i,\gamma} \leftarrow \sum_{w \in D} \frac{1}{2} {}^2D^2_{i,w} \tau^{11}_{\gamma,w,i} \quad (2r_D r_T N_o) \quad (4470)$$

Raw expression

$${}^2R^2_{i,\epsilon} \leftarrow \sum_{\gamma \in A} \sum_{j \in O} \sum_{k \in O} \sum_{l \in O} \sum_{a \in V} \sum_{b \in V} \sum_{c \in V} \sum_{d \in V} \frac{1}{2} \quad (4471)$$

$$\begin{aligned} & {}^1T_{c,i} \quad {}^1T_{d,j} \quad Y^{1,*}_{a,\epsilon} \quad Z^*_{\epsilon,\gamma} \quad Y^{3,*}_{b,\gamma} \\ & Y^{4,*}_{j,\gamma} \quad {}^2D^{a,i,b,j} \quad {}^2T_{a,k,b,l} \quad V_{k,c,l,d} \end{aligned}$$



Factorized expression

$$\tau_{\gamma,w,i}^0 = \sum_{a \in V} {}^2D_{a,w}^1 T_{a,i} Y_{a,\gamma}^{1,*} \quad (3r_D r_T N_o N_v) \quad (4472)$$

$$\tau_{\gamma,\alpha}^1 = \sum_{a \in V} W_{a,\alpha}^2 Y_{a,\gamma}^3 \quad (2r_T r_V N_v) \quad (4473)$$

$$\tau_{\gamma,\alpha,i}^2 = \sum_{\delta \in A} Z_{\gamma,\delta} Y_{i,\delta}^4 \tau_{\delta,\alpha}^1 \quad (3r_T^2 r_V N_o) \quad (4474)$$

$$\tau_{\gamma,\delta,w}^3 = \sum_{a \in V} {}^2D_{a,w}^3 Y_{a,\gamma}^1 Y_{a,\delta}^{3,*} \quad (3r_D r_T^2 N_v) \quad (4475)$$

$$\tau_{\alpha,i}^4 = \sum_{a \in V} {}^1T_{a,i} W_{a,\alpha}^4 \quad (2r_V N_o N_v) \quad (4476)$$

$$\tau_{\alpha,i,j}^5 = \sum_{\beta \in B} X_{\alpha,\beta} W_{j,\beta}^3 \tau_{\beta,i}^4 \quad (3r_V^2 N_o^2) \quad (4477)$$

$$\tau_{\gamma,\alpha,i}^6 = \sum_{j \in O} Y_{j,\gamma}^2 \tau_{\alpha,i,j}^5 \quad (2r_T r_V N_o^2) \quad (4478)$$

$$\tau_{\gamma,\delta,\alpha,w}^7 = \sum_{i \in O} {}^2D_{i,w}^4 Y_{i,\delta}^{4,*} \tau_{\gamma,\delta,w}^3 \tau_{\gamma,\alpha,i}^6 \quad (4r_D r_T^2 r_V N_o) \quad (4479)$$

$$\tau_{\gamma,\alpha,w,i}^8 = \sum_{\delta \in A} \tau_{\delta,\alpha,i}^2 \tau_{\delta,\gamma,\alpha,w}^7 \quad (2r_D r_T^2 r_V N_o) \quad (4480)$$

$$\tau_{\gamma,w,i,j}^9 = \sum_{\alpha \in B} W_{i,\alpha}^1 \tau_{\gamma,\alpha,w,j}^8 \quad (2r_D r_T r_V N_o^2) \quad (4481)$$

$$\tau_{\gamma,w,i,j}^{10} = \sum_{\delta \in A} Z_{\gamma,\delta}^* \tau_{\delta,w,i,j}^9 \quad (2r_D r_T^2 N_o^2) \quad (4482)$$

$$\tau_{\gamma,w,i}^{11} = \sum_{j \in O} \tau_{\gamma,w,j}^0 \tau_{\gamma,w,j,i}^{10} \quad (2r_D r_T N_o^2) \quad (4483)$$

$${}^2R_{i,\gamma}^2 \leftarrow \sum_{w \in D} \frac{1}{2} {}^2D_{i,w}^2 \tau_{\gamma,w,i}^{11} \quad (2r_D r_T N_o) \quad (4484)$$

Raw expression

$${}^2R_{i,\epsilon}^2 \leftarrow \sum_{\gamma \in A} \sum_{j \in O} \sum_{k \in O} \sum_{l \in O} \sum_{a \in V} \sum_{b \in V} \sum_{c \in V} \sum_{d \in V} \frac{1}{2} \quad (4485)$$

$${}^1T_{c,i} {}^1T_{d,j} Y_{a,\epsilon}^{1,*} Z_{\epsilon,\gamma}^* Y_{b,\gamma}^{3,*} Y_{j,\gamma}^{4,*} {}^2D_{a,i,b,j} {}^2T_{b,k,a,l} V_{k,d,l,c}$$

Factorized expression

$$\tau_{\gamma,w,i}^0 = \sum_{a \in V} {}^2D_{a,w}^1 T_{a,i} Y_{a,\gamma}^{1,*} \quad (3r_D r_T N_o N_v) \quad (4486)$$

$$\tau_{\gamma,\alpha}^1 = \sum_{a \in V} W_{a,\alpha}^2 Y_{a,\gamma}^1 \quad (2r_T r_V N_v) \quad (4487)$$

$$\tau_{\gamma,\alpha,i}^2 = \sum_{\delta \in A} Y_{i,\delta}^2 Z_{\delta,\gamma} \tau_{\delta,\alpha}^1 \quad (3r_T^2 r_V N_o) \quad (4488)$$

$$\tau_{\gamma,\delta,w}^3 = \sum_{a \in V} {}^2D_{a,w}^3 Y_{a,\gamma}^3 Y_{a,\delta}^{3,*} \quad (3r_D r_T^2 N_v) \quad (4489)$$

$$\tau_{\alpha,i}^4 = \sum_{a \in V} {}^1T_{a,i} W_{a,\alpha}^4 \quad (2r_V N_o N_v) \quad (4490)$$

$$\tau_{\alpha,i,j}^5 = \sum_{\beta \in B} X_{\alpha,\beta} W_{j,\beta}^3 \tau_{\beta,i}^4 \quad (3r_V^2 N_o^2) \quad (4491)$$

$$\tau_{\gamma,\alpha,i}^6 = \sum_{j \in O} Y_{j,\gamma}^4 \tau_{\alpha,i,j}^5 \quad (2r_T r_V N_o^2) \quad (4492)$$

$$\tau_{\gamma,\delta,\alpha,w}^7 = \sum_{i \in O} {}^2D_{i,w}^4 Y_{i,\delta}^{4,*} \tau_{\gamma,\delta,w}^3 \tau_{\gamma,\alpha,i}^6 \quad (4r_D r_T^2 r_V N_o) \quad (4493)$$

$$\tau_{\gamma,\alpha,w,i}^8 = \sum_{\delta \in A} \tau_{\delta,\alpha,i}^2 \tau_{\delta,\gamma,\alpha,w}^7 \quad (2r_D r_T^2 r_V N_o) \quad (4494)$$

$$\tau_{\gamma,w,i,j}^9 = \sum_{\alpha \in B} W_{i,\alpha}^1 \tau_{\gamma,\alpha,w,j}^8 \quad (2r_D r_T r_V N_o^2) \quad (4495)$$

$$\tau_{\gamma,w,i,j}^{10} = \sum_{\delta \in A} Z_{\gamma,\delta}^* \tau_{\delta,w,i,j}^9 \quad (2r_D r_T^2 N_o^2) \quad (4496)$$

$$\tau_{\gamma,w,i}^{11} = \sum_{j \in O} \tau_{\gamma,w,j}^0 \tau_{\gamma,w,j,i}^{10} \quad (2r_D r_T N_o^2) \quad (4497)$$

$${}^2R^2_{i,\gamma} \leftarrow \sum_{w \in D} \frac{1}{2} {}^2D^2_{i,w} \tau^{11}_{\gamma,w,i} \quad (2r_D r_T N_o) \quad (4498)$$

Raw expression

$${}^2R^2_{i,\epsilon} \leftarrow \sum_{\gamma \in A} \sum_{j \in O} \sum_{k \in O} \sum_{l \in O} \sum_{a \in V} \sum_{b \in V} \sum_{c \in V} \sum_{d \in V} \frac{1}{2} \quad (4499)$$

$${}^1T_{c,i} \quad {}^1T_{d,k} \quad Y^{1,*}_{a,\epsilon} \quad Z^{*,\epsilon}_{\gamma} \quad Y^{3,*}_{b,\gamma}$$

$$Y^{4,*}_{j,\gamma} \quad {}^2D^{a,i,b,j} \quad {}^2T_{a,l,b,j} \quad V_{k,c,l,d}$$

Factorized expression

$$\tau^0_{\gamma,\delta,w} = \sum_{a \in V} {}^2D^3_{a,w} Y^1_{a,\gamma} Y^{3,*}_{a,\delta} \quad (3r_D r_T^2 N_v) \quad (4500)$$

$$\tau^1_{\gamma,\delta,w} = \sum_{i \in O} {}^2D^4_{i,w} Y^2_{i,\gamma} Y^{4,*}_{i,\delta} \quad (3r_D r_T^2 N_o) \quad (4501)$$

$$\tau^2_{\gamma,\delta,w} = \sum_{\epsilon \in A} Z^{*,\epsilon}_{\delta} \tau^0_{\gamma,\epsilon,w} \tau^1_{\gamma,\epsilon,w} \quad (3r_D r_T^3) \quad (4502)$$

$$\tau^3_{\gamma,\delta,w} = \sum_{\epsilon \in A} Z_{\epsilon,\gamma} \tau^2_{\epsilon,\delta,w} \quad (2r_D r_T^3) \quad (4503)$$

$$\tau^4_{\gamma,w,i} = \sum_{a \in V} {}^2D^1_{a,w} {}^1T_{a,i} Y^{1,*}_{a,\gamma} \quad (3r_D r_T N_o N_v) \quad (4504)$$

$$\tau^5_{\alpha,i} = \sum_{a \in V} {}^1T_{a,i} W^2_{a,\alpha} \quad (2r_V N_o N_v) \quad (4505)$$

$$\tau^6_{\alpha,\beta} = \sum_{i \in O} W^3_{i,\beta} \tau^5_{\alpha,i} \quad (2r_V^2 N_o) \quad (4506)$$

$$\tau^7_{\alpha,i} = \sum_{\beta \in B} W^1_{i,\beta} X_{\beta,\alpha} \tau^6_{\beta,\alpha} \quad (3r_V^2 N_o) \quad (4507)$$

$$\tau^8_{i,a} = \sum_{\alpha \in B} W^4_{a,\alpha} \tau^7_{\alpha,i} \quad (2r_V N_o N_v) \quad (4508)$$

$$\tau^9_{\gamma,i} = \sum_{a \in V} Y^3_{a,\gamma} \tau^8_{i,a} \quad (2r_T N_o N_v) \quad (4509)$$

$$\tau^{10}_{\gamma,\delta,w} = \sum_{i \in O} \tau^9_{\gamma,i} \tau^4_{\delta,w,i} \quad (2r_D r_T^2 N_o) \quad (4510)$$

$${}^2R^2_{i,\gamma} \leftarrow \sum_{\delta \in A} \sum_{w \in D} \frac{1}{2} {}^2D^2_{i,w} Y^4_{i,\delta} \tau^{10}_{\delta,\gamma,w} \tau^3_{\delta,\gamma,w} \quad (4r_D r_T^2 N_o) \quad (4511)$$

Raw expression

$${}^2R^2_{i,\epsilon} \leftarrow \sum_{\gamma \in A} \sum_{j \in O} \sum_{k \in O} \sum_{l \in O} \sum_{a \in V} \sum_{b \in V} \sum_{c \in V} \sum_{d \in V} \frac{1}{2} \quad (4512)$$

$${}^1T_{c,i} \quad {}^1T_{d,k} \quad Y^{1,*}_{a,\epsilon} \quad Z^{*,\epsilon}_{\gamma} \quad Y^{3,*}_{b,\gamma}$$

$$Y^{4,*}_{j,\gamma} \quad {}^2D^{a,i,b,j} \quad {}^2T_{b,j,a,l} \quad V_{k,c,l,d}$$

Factorized expression

$$\tau^0_{\gamma,\delta,w} = \sum_{a \in V} {}^2D^3_{a,w} Y^3_{a,\gamma} Y^{3,*}_{a,\delta} \quad (3r_D r_T^2 N_v) \quad (4513)$$

$$\tau^1_{\gamma,\delta,w} = \sum_{i \in O} {}^2D^4_{i,w} Y^4_{i,\gamma} Y^{4,*}_{i,\delta} \quad (3r_D r_T^2 N_o) \quad (4514)$$

$$\tau^2_{\gamma,\delta,w} = \sum_{\epsilon \in A} Z^{*,\epsilon}_{\delta} \tau^0_{\gamma,\epsilon,w} \tau^1_{\gamma,\epsilon,w} \quad (3r_D r_T^3) \quad (4515)$$

$$\tau^3_{\gamma,\delta,w} = \sum_{\epsilon \in A} Z_{\gamma,\epsilon} \tau^2_{\epsilon,\delta,w} \quad (2r_D r_T^3) \quad (4516)$$

$$\tau^4_{\gamma,w,i} = \sum_{a \in V} {}^2D^1_{a,w} {}^1T_{a,i} Y^{1,*}_{a,\gamma} \quad (3r_D r_T N_o N_v) \quad (4517)$$

$$\tau^5_{\alpha,i} = \sum_{a \in V} {}^1T_{a,i} W^2_{a,\alpha} \quad (2r_V N_o N_v) \quad (4518)$$

$$\tau^6_{\alpha,\beta} = \sum_{i \in O} W^3_{i,\beta} \tau^5_{\alpha,i} \quad (2r_V^2 N_o) \quad (4519)$$

$$\tau^7_{\alpha,i} = \sum_{\beta \in B} W^1_{i,\beta} X_{\beta,\alpha} \tau^6_{\beta,\alpha} \quad (3r_V^2 N_o) \quad (4520)$$

$$\tau^8_{i,a} = \sum_{\alpha \in B} W^4_{a,\alpha} \tau^7_{\alpha,i} \quad (2r_V N_o N_v) \quad (4521)$$

$$\tau^9_{\gamma,i} = \sum_{a \in V} Y^1_{a,\gamma} \tau^8_{i,a} \quad (2r_T N_o N_v) \quad (4522)$$

$$\tau^{10}_{\gamma,\delta,w} = \sum_{i \in O} \tau^9_{\gamma,i} \tau^4_{\delta,w,i} \quad (2r_D r_T^2 N_o) \quad (4523)$$

$${}^2R^2_{i,\gamma} \leftarrow \sum_{\delta \in A} \sum_{w \in D} \frac{1}{2} {}^2D^2_{i,w} Y^2_{i,\delta} \tau^{10}_{\delta,\gamma,w} \tau^3_{\delta,\gamma,w} \quad (4r_D r_T^2 N_o) \quad (4524)$$

Raw expression

$${}^2R^2_{i,\epsilon} \leftarrow \sum_{\gamma \in A} \sum_{j \in O} \sum_{k \in O} \sum_{l \in O} \sum_{a \in V} \sum_{b \in V} \sum_{c \in V} \sum_{d \in V} \frac{1}{2} \quad (4525)$$

$${}^1T_{c,j} {}^1T_{d,k} Y^{1,*}_{a,\epsilon} Z^{*,\epsilon}_{\gamma} Y^{3,*}_{b,\gamma} Y^{4,*}_{j,\gamma} {}^2D^{a,i,b,j} {}^2T_{a,i,b,l} V_{k,c,l,d}$$

Factorized expression

$$\tau^0_{\gamma,\delta,w} = \sum_{a \in V} {}^2D^1_{a,w} Y^1_{a,\gamma} Y^{1,*}_{a,\delta} \quad (3r_D r_T^2 N_v) \quad (4526)$$

$$\tau^1_{\alpha,i} = \sum_{a \in V} {}^1T_{a,i} W^4_{a,\alpha} \quad (2r_V N_o N_v) \quad (4527)$$

$$\tau^2_{\alpha,i,j} = \sum_{\beta \in B} X_{\alpha,\beta} W^3_{j,\beta} \tau^1_{\beta,i} \quad (3r_V^2 N_o^2) \quad (4528)$$

$$\tau^3_{\gamma,\alpha,i} = \sum_{j \in O} Y^2_{j,\gamma} \tau^2_{\alpha,i,j} \quad (2r_T r_V N_o^2) \quad (4529)$$

$$\tau^4_{\gamma,w,i} = \sum_{a \in V} {}^2D^3_{a,w} {}^1T_{a,i} Y^{3,*}_{a,\gamma} \quad (3r_D r_T N_o N_v) \quad (4530)$$

$$\tau^5_{\gamma,w,i,j} = \sum_{\delta \in A} {}^2D^4_{i,w} Z^{*,\gamma}_{\delta} Y^{4,*}_{i,\delta} \tau^4_{\delta,w,j} \quad (4r_D r_T^2 N_o^2) \quad (4531)$$

$$\tau^6_{\gamma,\alpha,w,i} = \sum_{j \in O} W^1_{j,\alpha} \tau^5_{\gamma,w,i,j} \quad (2r_D r_T r_V N_o^2) \quad (4532)$$

$$\tau^7_{\gamma,\alpha} = \sum_{a \in V} W^2_{a,\alpha} Y^3_{a,\gamma} \quad (2r_T r_V N_v) \quad (4533)$$

$$\tau^8_{\gamma,\alpha,i} = \sum_{\delta \in A} Z_{\gamma,\delta} Y^4_{i,\delta} \tau^7_{\delta,\alpha} \quad (3r_T^2 r_V N_o) \quad (4534)$$

$$\tau^9_{\gamma,\delta,\alpha,w} = \sum_{i \in O} \tau^8_{\gamma,\alpha,i} \tau^6_{\delta,\alpha,w,i} \quad (2r_D r_T^2 r_V N_o) \quad (4535)$$

$$\tau^{10}_{\gamma,\delta,w,i} = \sum_{\alpha \in B} \tau^3_{\gamma,\alpha,i} \tau^9_{\gamma,\delta,\alpha,w} \quad (2r_D r_T^2 r_V N_o) \quad (4536)$$

$$\tau^{11}_{\gamma,w,i} = \sum_{\delta \in A} \tau^0_{\delta,\gamma,w} \tau^{10}_{\delta,\gamma,w,i} \quad (2r_D r_T^2 N_o) \quad (4537)$$

$${}^2R^2_{i,\gamma} \leftarrow \sum_{w \in D} \frac{1}{2} {}^2D^2_{i,w} \tau^{11}_{\gamma,w,i} \quad (2r_D r_T N_o) \quad (4538)$$

Raw expression

$${}^2R^2_{i,\epsilon} \leftarrow \sum_{\gamma \in A} \sum_{j \in O} \sum_{k \in O} \sum_{l \in O} \sum_{a \in V} \sum_{b \in V} \sum_{c \in V} \sum_{d \in V} \frac{1}{2} \quad (4539)$$

$${}^1T_{c,j} {}^1T_{d,k} Y^{1,*}_{a,\epsilon} Z^{*,\epsilon}_{\gamma} Y^{3,*}_{b,\gamma} Y^{4,*}_{j,\gamma} {}^2D^{a,i,b,j} {}^2T_{b,l,a,i} V_{k,c,l,d}$$

Factorized expression

$$\tau^0_{\alpha,i} = \sum_{a \in V} {}^1T_{a,i} W^4_{a,\alpha} \quad (2r_V N_o N_v) \quad (4540)$$

$$\tau^1_{\alpha,i,j} = \sum_{\beta \in B} X_{\alpha,\beta} W^3_{j,\beta} \tau^0_{\beta,i} \quad (3r_V^2 N_o^2) \quad (4541)$$

$$\tau^2_{\gamma,\alpha,i} = \sum_{j \in O} Y^4_{j,\gamma} \tau^1_{\alpha,i,j} \quad (2r_T r_V N_o^2) \quad (4542)$$

$$\tau^3_{\gamma,w,i} = \sum_{a \in V} {}^2D^3_{a,w} {}^1T_{a,i} Y^{3,*}_{a,\gamma} \quad (3r_D r_T N_o N_v) \quad (4543)$$

$$\tau^4_{\gamma,w,i,j} = \sum_{\delta \in A} {}^2D^4_{i,w} Z^{*,\gamma}_{\delta} Y^{4,*}_{i,\delta} \tau^3_{\delta,w,j} \quad (4r_D r_T^2 N_o^2) \quad (4544)$$

$$\tau^5_{\gamma,\alpha,w,i} = \sum_{j \in O} W^1_{j,\alpha} \tau^4_{\gamma,w,i,j} \quad (2r_D r_T r_V N_o^2) \quad (4545)$$

$$\tau^6_{\gamma,\alpha} = \sum_{a \in V} W^2_{a,\alpha} Y^1_{a,\gamma} \quad (2r_T r_V N_v) \quad (4546)$$

$$\tau^7_{\gamma,\alpha,i} = \sum_{\delta \in A} Y^2_{i,\delta} Z_{\delta,\gamma} \tau^6_{\delta,\alpha} \quad (3r_T^2 r_V N_o) \quad (4547)$$

$$\tau^8_{\gamma,\delta,\alpha,w} = \sum_{i \in O} \tau^7_{\gamma,\alpha,i} \tau^5_{\delta,\alpha,w,i} \quad (2r_D r_T^2 r_V N_o) \quad (4548)$$

$$\tau^9_{\gamma,\delta,w,i} = \sum_{\alpha \in B} \tau^2_{\gamma,\alpha,i} \tau^8_{\gamma,\delta,\alpha,w} \quad (2r_D r_T^2 r_V N_o) \quad (4549)$$

$$\tau^8_{\gamma,\alpha,w} = \sum_{\beta \in B} X_{\beta,\alpha} \tau^5_{\gamma,\beta,w} \tau^7_{\gamma,\beta,w} \quad (3r_D r_T r_V^2) \quad (4562)$$

$$\tau^{10}_{\gamma,\delta,w} = \sum_{a \in V} {}^2D^1_{a,w} Y^3_{a,\gamma} Y^{1,*}_{a,\delta} \quad (3r_D r_T^2 N_v) \quad (4550)$$

$$\tau^9_{\gamma,\alpha,w} = \sum_{\delta \in A} Z^*_{\gamma,\delta} \tau^8_{\delta,\alpha,w} \quad (2r_D r_T^2 r_V) \quad (4563)$$

$$\tau^{11}_{\gamma,w,i} = \sum_{\delta \in A} \tau^{10}_{\delta,\gamma,w} \tau^9_{\delta,\gamma,w,i} \quad (2r_D r_T^2 N_o) \quad (4551)$$

$$\tau^{10}_{\gamma,\delta,w,i} = \sum_{\alpha \in B} \tau^1_{\gamma,\alpha} \tau^3_{\gamma,\alpha,i} \tau^9_{\delta,\alpha,w} \quad (3r_D r_T^2 r_V N_o) \quad (4564)$$

$${}^2R^2_{i,\gamma} \leftarrow \sum_{w \in D} \frac{1}{2} {}^2D^2_{i,w} \tau^{11}_{\gamma,w,i} \quad (2r_D r_T N_o) \quad (4552)$$

$$\tau^{11}_{\gamma,w,i} = \sum_{\delta \in A} \tau^0_{\delta,\gamma,w} \tau^{10}_{\delta,\gamma,w,i} \quad (2r_D r_T^2 N_o) \quad (4565)$$

Raw expression

$${}^2R^2_{i,\epsilon} \leftarrow - \sum_{\gamma \in A} \sum_{j \in O} \sum_{k \in O} \sum_{l \in O} \sum_{a \in V} \sum_{b \in V} \sum_{c \in V} \sum_{d \in V} {}^1T_{a,k} \\ {}^1T_{c,i} Y^{1,*}_{a,\epsilon} Z^*_{\epsilon,\gamma} Y^{3,*}_{b,\gamma} \\ Y^{4,*}_{j,\gamma} {}^2D^{a,i,b,j} {}^2T_{b,j,d,l} V_{k,c,l,d} \quad (4553)$$

$${}^2R^2_{i,\gamma} \leftarrow \sum_{w \in D} \frac{1}{2} {}^2D^2_{i,w} \tau^{11}_{\gamma,w,i} \quad (2r_D r_T N_o) \quad (4566)$$

Raw expression

$${}^2R^2_{i,\epsilon} \leftarrow - \sum_{\gamma \in A} \sum_{j \in O} \sum_{k \in O} \sum_{l \in O} \sum_{a \in V} \sum_{b \in V} \sum_{c \in V} \sum_{d \in V} {}^1T_{a,k} \\ {}^1T_{c,i} Y^{1,*}_{a,\epsilon} Z^*_{\epsilon,\gamma} Y^{3,*}_{b,\gamma} \\ Y^{4,*}_{j,\gamma} {}^2D^{a,i,b,j} {}^2T_{d,l,b,j} V_{k,c,l,d} \quad (4567)$$

Factorized expression

$$\tau^0_{\gamma,\delta,w} = \sum_{a \in V} {}^2D^1_{a,w} Y^1_{a,\gamma} Y^{1,*}_{a,\delta} \quad (3r_D r_T^2 N_v) \quad (4554)$$

Factorized expression

$$\tau^0_{\gamma,\delta,w} = \sum_{a \in V} {}^2D^1_{a,w} Y^3_{a,\gamma} Y^{1,*}_{a,\delta} \quad (3r_D r_T^2 N_v) \quad (4568)$$

$$\tau^1_{\gamma,\alpha} = \sum_{i \in O} W^3_{i,\alpha} Y^2_{i,\gamma} \quad (2r_T r_V N_o) \quad (4555)$$

$$\tau^1_{\gamma,\alpha} = \sum_{a \in V} W^4_{a,\alpha} Y^1_{a,\gamma} \quad (2r_T r_V N_v) \quad (4569)$$

$$\tau^2_{\gamma,\alpha} = \sum_{a \in V} W^4_{a,\alpha} Y^3_{a,\gamma} \quad (2r_T r_V N_v) \quad (4556)$$

$$\tau^2_{\gamma,\alpha,i} = \sum_{\delta \in A} Y^2_{i,\delta} Z_{\delta,\gamma} \tau^1_{\delta,\alpha} \quad (3r_T^2 r_V N_o) \quad (4570)$$

$$\tau^3_{\gamma,\alpha,i} = \sum_{\delta \in A} Z_{\gamma,\delta} Y^4_{i,\delta} \tau^2_{\delta,\alpha} \quad (3r_T^2 r_V N_o) \quad (4557)$$

$$\tau^3_{\gamma,\alpha} = \sum_{i \in O} W^3_{i,\alpha} Y^4_{i,\gamma} \quad (2r_T r_V N_o) \quad (4571)$$

$$\tau^4_{\alpha,i} = \sum_{a \in V} {}^1T_{a,i} W^2_{a,\alpha} \quad (2r_V N_o N_v) \quad (4558)$$

$$\tau^4_{\alpha,i} = \sum_{a \in V} {}^1T_{a,i} W^2_{a,\alpha} \quad (2r_V N_o N_v) \quad (4572)$$

$$\tau^5_{\gamma,\alpha,w} = \sum_{i \in O} {}^2D^4_{i,w} Y^{4,*}_{i,\gamma} \tau^4_{\alpha,i} \quad (3r_D r_T r_V N_o) \quad (4559)$$

$$\tau^5_{\gamma,\alpha,w} = \sum_{i \in O} {}^2D^4_{i,w} Y^{4,*}_{i,\gamma} \tau^4_{\alpha,i} \quad (3r_D r_T r_V N_o) \quad (4573)$$

$$\tau^6_{\gamma,w,i} = \sum_{a \in V} {}^2D^3_{a,w} {}^1T_{a,i} Y^{3,*}_{a,\gamma} \quad (3r_D r_T N_o N_v) \quad (4560)$$

$$\tau^6_{\gamma,w,i} = \sum_{a \in V} {}^2D^3_{a,w} {}^1T_{a,i} Y^{3,*}_{a,\gamma} \quad (3r_D r_T N_o N_v) \quad (4574)$$

$$\tau^7_{\gamma,\alpha,w} = \sum_{i \in O} W^1_{i,\alpha} \tau^6_{\gamma,w,i} \quad (2r_D r_T r_V N_o) \quad (4561)$$

$$\tau^7_{\gamma,\alpha,w} = \sum_{i \in O} W^1_{i,\alpha} \tau^6_{\gamma,w,i} \quad (2r_D r_T r_V N_o) \quad (4575)$$

$$\tau^6_{\gamma,i,j} = \sum_{\alpha \in B} W^1_{j,\alpha} \tau^2_{\gamma,\alpha} \tau^5_{\gamma,\alpha,i} \quad (3r_T r_V N_o^2) \quad (4588)$$

$$\tau^8_{\gamma,\alpha,w} = \sum_{\beta \in B} X_{\beta,\alpha} \tau^5_{\gamma,\beta,w} \tau^7_{\gamma,\beta,w} \quad (3r_D r_T r_V^2) \quad (4576)$$

$$\tau^7_{\gamma,i,j} = \sum_{\delta \in A} Z_{\gamma,\delta} \tau^6_{\delta,i,j} \quad (2r_T^2 N_o^2) \quad (4589)$$

$$\tau^9_{\gamma,\alpha,w} = \sum_{\delta \in A} Z^*_{\gamma,\delta} \tau^8_{\delta,\alpha,w} \quad (2r_D r_T^2 r_V) \quad (4577)$$

$$\tau^8_{\gamma,\delta,w} = \sum_{i \in O} \sum_{j \in O} {}^2D^4_{i,w} Y^{4,*}_{i,\delta} \tau^1_{\delta,w,j} \tau^7_{\gamma,i,j} \quad (4r_D r_T^2 N_o^2) \quad (4590)$$

$$\tau^{10}_{\gamma,\delta,w,i} = \sum_{\alpha \in B} \tau^3_{\gamma,\alpha} \tau^2_{\gamma,\alpha,i} \tau^9_{\delta,\alpha,w} \quad (3r_D r_T^2 r_V N_o) \quad (4578)$$

$$\tau^9_{\gamma,\delta,w} = \sum_{\epsilon \in A} Z^*_{\delta,\epsilon} \tau^8_{\gamma,\epsilon,w} \quad (2r_D r_T^3) \quad (4591)$$

$$\tau^{11}_{\gamma,w,i} = \sum_{\delta \in A} \tau^0_{\delta,\gamma,w} \tau^{10}_{\delta,\gamma,w,i} \quad (2r_D r_T^2 N_o) \quad (4579)$$

$${}^2R^2_{i,\gamma} \leftarrow \sum_{\delta \in A} \sum_{w \in D} \frac{1}{2} {}^2D^2_{i,w} Y^2_{i,\delta} \tau^0_{\delta,\gamma,w} \tau^9_{\delta,\gamma,w} \quad (4r_D r_T^2 N_o) \quad (4592)$$

$${}^2R^2_{i,\gamma} \leftarrow \sum_{w \in D} \frac{1}{2} {}^2D^2_{i,w} \tau^{11}_{\gamma,w,i} \quad (2r_D r_T N_o) \quad (4580)$$

Raw expression

$${}^2R^2_{i,\epsilon} \leftarrow - \sum_{\gamma \in A} \sum_{j \in O} \sum_{k \in O} \sum_{l \in O} \sum_{a \in V} \sum_{b \in V} \sum_{c \in V} \sum_{d \in V} {}^1T_{a,k} \\ {}^1T_{c,l} Y^{1,*}_{a,\epsilon} Z^*_{\epsilon,\gamma} Y^{3,*}_{b,\gamma} Y^{4,*}_{j,\gamma} {}^2D^{a,i,b,j} {}^2T_{b,j,d,i} V_{k,d,l,c} \quad (4581)$$

Factorized expression

$$\tau^0_{\gamma,\delta,w} = \sum_{a \in V} {}^2D^1_{a,w} Y^1_{a,\gamma} Y^{1,*}_{a,\delta} \quad (3r_D r_T^2 N_v) \quad (4582)$$

$$\tau^1_{\gamma,w,i} = \sum_{a \in V} {}^2D^3_{a,w} {}^1T_{a,i} Y^{3,*}_{a,\gamma} \quad (3r_D r_T N_o N_v) \quad (4583)$$

$$\tau^2_{\gamma,\alpha} = \sum_{a \in V} W^2_{a,\alpha} Y^3_{a,\gamma} \quad (2r_T r_V N_v) \quad (4584)$$

$$\tau^3_{\alpha,i} = \sum_{a \in V} {}^1T_{a,i} W^4_{a,\alpha} \quad (2r_V N_o N_v) \quad (4585)$$

$$\tau^4_{\alpha,i,j} = \sum_{\beta \in B} X_{\alpha,\beta} W^3_{j,\beta} \tau^3_{\beta,i} \quad (3r_V^2 N_o^2) \quad (4586)$$

$$\tau^5_{\gamma,\alpha,i} = \sum_{j \in O} Y^4_{j,\gamma} \tau^4_{\alpha,i,j} \quad (2r_T r_V N_o^2) \quad (4587)$$

Raw expression

$${}^2R^2_{i,\epsilon} \leftarrow - \sum_{\gamma \in A} \sum_{j \in O} \sum_{k \in O} \sum_{l \in O} \sum_{a \in V} \sum_{b \in V} \sum_{c \in V} \sum_{d \in V} {}^1T_{a,k} \\ {}^1T_{c,l} Y^{1,*}_{a,\epsilon} Z^*_{\epsilon,\gamma} Y^{3,*}_{b,\gamma} Y^{4,*}_{j,\gamma} {}^2D^{a,i,b,j} {}^2T_{d,i,b,j} V_{k,d,l,c} \quad (4593)$$

Factorized expression

$$\tau^0_{\gamma,\delta,w} = \sum_{a \in V} {}^2D^1_{a,w} Y^3_{a,\gamma} Y^{1,*}_{a,\delta} \quad (3r_D r_T^2 N_v) \quad (4594)$$

$$\tau^1_{\gamma,w,i} = \sum_{a \in V} {}^2D^3_{a,w} {}^1T_{a,i} Y^{3,*}_{a,\gamma} \quad (3r_D r_T N_o N_v) \quad (4595)$$

$$\tau^2_{\gamma,\alpha} = \sum_{a \in V} W^2_{a,\alpha} Y^1_{a,\gamma} \quad (2r_T r_V N_v) \quad (4596)$$

$$\tau^3_{\alpha,i} = \sum_{a \in V} {}^1T_{a,i} W^4_{a,\alpha} \quad (2r_V N_o N_v) \quad (4597)$$

$$\tau^4_{\alpha,i,j} = \sum_{\beta \in B} X_{\alpha,\beta} W^3_{j,\beta} \tau^3_{\beta,i} \quad (3r_V^2 N_o^2) \quad (4598)$$

$$\tau^5_{\gamma,\alpha,i} = \sum_{j \in O} Y^2_{j,\gamma} \tau^4_{\alpha,i,j} \quad (2r_T r_V N_o^2) \quad (4599)$$

$$\tau_{\gamma,i,j}^6 = \sum_{\alpha \in B} W_{j,\alpha}^1 \tau_{\gamma,\alpha}^2 \tau_{\gamma,\alpha,i}^5 \quad (3r_T r_V N_o^2) \quad (4600)$$

$$\tau_{i,a}^6 = \sum_{\alpha \in B} W_{a,\alpha}^4 \tau_{\alpha,i}^5 \quad (2r_V N_o N_v) \quad (4612)$$

$$\tau_{\gamma,i,j}^7 = \sum_{\delta \in A} Z_{\delta,\gamma} \tau_{\delta,i,j}^6 \quad (2r_T^2 N_o^2) \quad (4601)$$

$$\tau_{\gamma,i}^7 = \sum_{a \in V} Y_{a,\gamma}^3 \tau_{i,a}^6 \quad (2r_T N_o N_v) \quad (4613)$$

$$\tau_{\gamma,\delta,w}^8 = \sum_{i \in O} \sum_{j \in O} {}^2D_{i,w}^4 Y_{i,\delta}^{4,*} \tau_{\delta,w,j}^1 \tau_{\gamma,i,j}^7 \quad (4r_D r_T^2 N_o^2) \quad (4602)$$

$$\tau_{\gamma,\delta,w}^8 = \sum_{i \in O} \tau_{\gamma,i}^7 \tau_{\delta,w,i}^2 \quad (2r_D r_T^2 N_o) \quad (4614)$$

$$\tau_{\gamma,\delta,w}^9 = \sum_{\epsilon \in A} Z_{\delta,\epsilon}^* \tau_{\gamma,\epsilon,w}^8 \quad (2r_D r_T^3) \quad (4603)$$

$$\tau_{\gamma,\delta,w}^9 = \sum_{\epsilon \in A} Z_{\delta,\epsilon}^* \tau_{\gamma,\epsilon,w}^1 \tau_{\gamma,\epsilon,w}^8 \quad (3r_D r_T^3) \quad (4615)$$

$$\tau_{\gamma,\delta,w}^{10} = \sum_{\epsilon \in A} Z_{\gamma,\epsilon} \tau_{\epsilon,\delta,w}^9 \quad (2r_D r_T^3) \quad (4616)$$

$${}^2R_{i,\gamma}^2 \leftarrow \sum_{\delta \in A} \sum_{w \in D} \frac{1}{2} {}^2D_{i,w}^2 Y_{i,\delta}^4 \tau_{\delta,\gamma,w}^0 \tau_{\delta,\gamma,w}^9 \quad (4r_D r_T^2 N_o) \quad (4604)$$

$${}^2R_{i,\gamma}^2 \leftarrow \sum_{\delta \in A} \sum_{w \in D} \frac{1}{2} {}^2D_{i,w}^2 Y_{i,\delta}^2 \tau_{\delta,\gamma,w}^0 \tau_{\delta,\gamma,w}^{10} \quad (4r_D r_T^2 N_o) \quad (4617)$$

Raw expression

$${}^2R_{i,\epsilon}^2 \leftarrow - \sum_{\gamma \in A} \sum_{j \in O} \sum_{k \in O} \sum_{l \in O} \sum_{a \in V} \sum_{b \in V} \sum_{c \in V} \sum_{d \in V} {}^1T_{b,k} \\ {}^1T_{c,j} Y_{a,\epsilon}^{1,*} Z_{\epsilon,\gamma}^* Y_{b,\gamma}^{3,*} \\ Y_{j,\gamma}^{4,*} {}^2D_{a,i,b,j} {}^2T_{a,i,d,l} V_{k,c,l,d} \quad (4605)$$

Factorized expression

$$\tau_{\gamma,\delta,w}^0 = \sum_{a \in V} {}^2D_{a,w}^1 Y_{a,\gamma}^1 Y_{a,\delta}^{1,*} \quad (3r_D r_T^2 N_v) \quad (4606)$$

$$\tau_{\gamma,\delta,w}^1 = \sum_{i \in O} {}^2D_{i,w}^4 Y_{i,\gamma}^4 Y_{i,\delta}^{4,*} \quad (3r_D r_T^2 N_o) \quad (4607)$$

$$\tau_{\gamma,w,i}^2 = \sum_{a \in V} {}^2D_{a,w}^3 {}^1T_{a,i} Y_{a,\gamma}^{3,*} \quad (3r_D r_T N_o N_v) \quad (4608)$$

$$\tau_{\alpha,i}^3 = \sum_{a \in V} {}^1T_{a,i} W_{a,\alpha}^2 \quad (2r_V N_o N_v) \quad (4609)$$

$$\tau_{\alpha,\beta}^4 = \sum_{i \in O} W_{i,\beta}^3 X_{\beta,\alpha} \tau_{\alpha,i}^3 \quad (2r_V^2 N_o) \quad (4610)$$

$$\tau_{\alpha,i}^5 = \sum_{\beta \in B} W_{i,\beta}^1 X_{\beta,\alpha} \tau_{\beta,\alpha}^4 \quad (3r_V^2 N_o) \quad (4611)$$

Raw expression

$${}^2R_{i,\epsilon}^2 \leftarrow - \sum_{\gamma \in A} \sum_{j \in O} \sum_{k \in O} \sum_{l \in O} \sum_{a \in V} \sum_{b \in V} \sum_{c \in V} \sum_{d \in V} {}^1T_{b,k} \\ {}^1T_{c,j} Y_{a,\epsilon}^{1,*} Z_{\epsilon,\gamma}^* Y_{b,\gamma}^{3,*} \\ Y_{j,\gamma}^{4,*} {}^2D_{a,i,b,j} {}^2T_{d,l,a,i} V_{k,c,l,d} \quad (4618)$$

Factorized expression

$$\tau_{\gamma,\delta,w}^0 = \sum_{a \in V} {}^2D_{a,w}^1 Y_{a,\gamma}^3 Y_{a,\delta}^{1,*} \quad (3r_D r_T^2 N_v) \quad (4619)$$

$$\tau_{\gamma,\delta,w}^1 = \sum_{i \in O} {}^2D_{i,w}^4 Y_{i,\gamma}^2 Y_{i,\delta}^{4,*} \quad (3r_D r_T^2 N_o) \quad (4620)$$

$$\tau_{\gamma,w,i}^2 = \sum_{a \in V} {}^2D_{a,w}^3 {}^1T_{a,i} Y_{a,\gamma}^{3,*} \quad (3r_D r_T N_o N_v) \quad (4621)$$

$$\tau_{\alpha,i}^3 = \sum_{a \in V} {}^1T_{a,i} W_{a,\alpha}^2 \quad (2r_V N_o N_v) \quad (4622)$$

$$\tau_{\alpha,\beta}^4 = \sum_{i \in O} W_{i,\beta}^3 \tau_{\alpha,i}^3 \quad (2r_V^2 N_o) \quad (4623)$$

$$\tau_{\alpha,i}^5 = \sum_{\beta \in B} W_{i,\beta}^1 X_{\beta,\alpha} \tau_{\beta,\alpha}^4 \quad (3r_V^2 N_o) \quad (4624)$$

$$\tau_{i,a}^6 = \sum_{\alpha \in B} W_{a,\alpha}^4 \tau_{\alpha,i}^5 \quad (2r_V N_o N_v) \quad (4625)$$

$$\tau_{\alpha,i}^6 = \sum_{a \in V} {}^1T_{a,i} W_{a,\alpha}^2 \quad (2r_V N_o N_v) \quad (4638)$$

$$\tau_{\gamma,i}^7 = \sum_{a \in V} Y_{a,\gamma}^1 \tau_{i,a}^6 \quad (2r_T N_o N_v) \quad (4626)$$

$$\tau_{\alpha,i,j}^7 = \sum_{\beta \in B} W_{j,\beta}^1 X_{\beta,\alpha} \tau_{\beta,i}^6 \quad (3r_V^2 N_o^2) \quad (4639)$$

$$\tau_{\gamma,\delta,w}^8 = \sum_{i \in O} \tau_{\gamma,i}^7 \tau_{\delta,w,i}^2 \quad (2r_D r_T^2 N_o) \quad (4627)$$

$$\tau_{\gamma,\alpha,i}^8 = \sum_{j \in O} Y_{j,\gamma}^2 \tau_{\alpha,i,j}^7 \quad (2r_T r_V N_o^2) \quad (4640)$$

$$\tau_{\gamma,\delta,w}^9 = \sum_{\epsilon \in A} Z_{\delta,\epsilon}^* \tau_{\gamma,\epsilon,w}^1 \tau_{\epsilon,w}^8 \quad (3r_D r_T^3) \quad (4628)$$

$$\tau_{\gamma,\delta,w,i}^9 = \sum_{\alpha \in B} \tau_{\gamma,\alpha,i}^8 \tau_{\gamma,\delta,\alpha,w}^5 \quad (2r_D r_T^2 r_V N_o) \quad (4641)$$

$$\tau_{\gamma,\delta,w}^{10} = \sum_{\epsilon \in A} Z_{\epsilon,\gamma} \tau_{\epsilon,\delta,w}^9 \quad (2r_D r_T^3) \quad (4629)$$

$$\tau_{\gamma,\delta,i}^{10} = \sum_{\epsilon \in A} \sum_{w \in D} {}^2D_{i,w}^2 \tau_{\epsilon,\gamma,w}^0 \tau_{\epsilon,\delta,w,i}^9 \quad (3r_D r_T^3 N_o) \quad (4642)$$

$${}^2R_{i,\gamma}^2 \leftarrow \sum_{\delta \in A} \sum_{w \in D} \frac{1}{2} {}^2D_{i,w}^2 Y_{i,\delta}^4 \tau_{\delta,\gamma,w}^0 \tau_{\delta,\gamma,w}^{10} \quad (4r_D r_T^2 N_o) \quad (4630)$$

$${}^2R_{i,\gamma}^2 \leftarrow \sum_{\delta \in A} \frac{1}{2} Z_{\gamma,\delta}^* \tau_{\gamma,\delta,i}^{10} \quad (2r_T^2 N_o) \quad (4643)$$

Raw expression

$${}^2R_{i,\epsilon}^2 \leftarrow - \sum_{\gamma \in A} \sum_{j \in O} \sum_{k \in O} \sum_{l \in O} \sum_{a \in V} \sum_{b \in V} \sum_{c \in V} \sum_{d \in V} {}^1T_{b,k} \\ {}^1T_{c,l} Y_{a,\epsilon}^{1,*} Z_{\epsilon,\gamma}^* Y_{b,\gamma}^{3,*} \\ Y_{j,\gamma}^{4,*} {}^2D_{a,i,b,j} {}^2T_{a,i,d,j} V_{k,d,l,c} \quad (4631)$$

Raw expression

$${}^2R_{i,\epsilon}^2 \leftarrow - \sum_{\gamma \in A} \sum_{j \in O} \sum_{k \in O} \sum_{l \in O} \sum_{a \in V} \sum_{b \in V} \sum_{c \in V} \sum_{d \in V} {}^1T_{b,k} \\ {}^1T_{c,l} Y_{a,\epsilon}^{1,*} Z_{\epsilon,\gamma}^* Y_{b,\gamma}^{3,*} \\ Y_{j,\gamma}^{4,*} {}^2D_{a,i,b,j} {}^2T_{d,j,a,i} V_{k,d,l,c} \quad (4644)$$

Factorized expression

$$\tau_{\gamma,\delta,w}^0 = \sum_{a \in V} {}^2D_{a,w}^1 Y_{a,\gamma}^1 Y_{a,\delta}^{1,*} \quad (3r_D r_T^2 N_v) \quad (4632)$$

$$\tau_{\gamma,\delta,w}^0 = \sum_{a \in V} {}^2D_{a,w}^1 Y_{a,w}^3 Y_{a,\gamma}^1 Y_{a,\delta}^{1,*} \quad (3r_D r_T^2 N_v) \quad (4645)$$

$$\tau_{\alpha,i}^1 = \sum_{a \in V} {}^1T_{a,i} W_{a,\alpha}^4 \quad (2r_V N_o N_v) \quad (4633)$$

$$\tau_{\alpha,i}^1 = \sum_{a \in V} {}^1T_{a,i} W_{a,\alpha}^2 \quad (2r_V N_o N_v) \quad (4646)$$

$$\tau_{\gamma,\alpha,w}^2 = \sum_{i \in O} {}^2D_{i,w}^4 Y_{i,\gamma}^{4,*} \tau_{\alpha,i}^1 \quad (3r_D r_T r_V N_o) \quad (4634)$$

$$\tau_{\gamma,\alpha,w}^2 = \sum_{i \in O} {}^2D_{i,w}^4 Y_{i,w}^{4,*} \tau_{\alpha,i}^1 \quad (3r_D r_T r_V N_o) \quad (4647)$$

$$\tau_{\gamma,\delta,w}^3 = \sum_{a \in V} {}^2D_{a,w}^3 Y_{a,\gamma}^3 Y_{a,\delta}^{3,*} \quad (3r_D r_T^2 N_v) \quad (4635)$$

$$\tau_{\gamma,\delta,w}^3 = \sum_{a \in V} {}^2D_{a,w}^3 Y_{a,\gamma}^1 Y_{a,\delta}^{3,*} \quad (3r_D r_T^2 N_v) \quad (4648)$$

$$\tau_{\gamma,\delta,w,i}^4 = \sum_{\epsilon \in A} Z_{\gamma,\epsilon} Y_{i,\epsilon}^4 \tau_{\epsilon,\delta,w}^3 \quad (3r_D r_T^3 N_o) \quad (4636)$$

$$\tau_{\gamma,\delta,w,i}^4 = \sum_{\epsilon \in A} Y_{i,\epsilon}^2 Z_{\epsilon,\gamma} \tau_{\epsilon,\delta,w}^3 \quad (3r_D r_T^3 N_o) \quad (4649)$$

$$\tau_{\gamma,\delta,\alpha,w}^5 = \sum_{i \in O} W_{i,\alpha}^3 \tau_{\delta,\alpha,w}^2 \tau_{\gamma,\delta,w,i}^4 \quad (3r_D r_T^2 r_V N_o) \quad (4637)$$

$$\tau_{\gamma,\delta,\alpha,w}^5 = \sum_{i \in O} W_{i,\alpha}^1 \tau_{\delta,\alpha,w}^2 \tau_{\gamma,\delta,w,i}^4 \quad (3r_D r_T^2 r_V N_o) \quad (4650)$$

$$\tau_{\alpha,i}^6 = \sum_{a \in V} {}^1T_{a,i} W_{a,\alpha}^4 \quad (2r_V N_o N_v) \quad (4651)$$

$$\tau_{\alpha,\beta}^6 = \sum_{i \in O} W_{i,\alpha}^1 \tau_{\beta,i}^5 \quad (2r_V^2 N_o) \quad (4664)$$

$$\tau_{\alpha,i,j}^7 = \sum_{\beta \in B} X_{\alpha,\beta} W_{j,\beta}^3 \tau_{\beta,i}^6 \quad (3r_V^2 N_o^2) \quad (4652)$$

$$\tau_{\alpha,i}^7 = \sum_{\beta \in B} X_{\alpha,\beta} W_{i,\beta}^3 \tau_{\alpha,\beta}^6 \quad (3r_V^2 N_o) \quad (4665)$$

$$\tau_{\gamma,\alpha,i}^8 = \sum_{j \in O} Y_{j,\gamma}^4 \tau_{\alpha,i,j}^7 \quad (2r_T r_V N_o^2) \quad (4653)$$

$$\tau_{i,a}^8 = \sum_{\alpha \in B} W_{a,\alpha}^2 \tau_{\alpha,i}^7 \quad (2r_V N_o N_v) \quad (4666)$$

$$\tau_{\gamma,\delta,w,i}^9 = \sum_{\alpha \in B} \tau_{\gamma,\alpha,i}^8 \tau_{\gamma,\delta,\alpha,w}^5 \quad (2r_D r_T^2 r_V N_o) \quad (4654)$$

$$\tau_{i,j}^9 = \sum_{a \in V} {}^1T_{a,i} \tau_{j,a}^8 \quad (2N_o^2 N_v) \quad (4667)$$

$$\tau_{\gamma,\delta,i}^{10} = \sum_{\epsilon \in A} \sum_{w \in D} {}^2D_{i,w}^2 \tau_{\epsilon,\gamma,w}^0 \tau_{\epsilon,\delta,w,i}^9 \quad (3r_D r_T^3 N_o) \quad (4655)$$

$$\tau_{\gamma,i}^{10} = \sum_{j \in O} Y_{j,\gamma}^2 \tau_{i,j}^9 \quad (2r_T N_o^2) \quad (4668)$$

$${}^2R_{i,\gamma}^2 \leftarrow \sum_{\delta \in A} \frac{1}{2} Z_{\gamma,\delta}^* \tau_{\gamma,\delta,i}^{10} \quad (2r_T^2 N_o) \quad (4656)$$

$${}^2R_{i,\gamma}^2 \leftarrow \sum_{\delta \in A} \sum_{w \in D} \frac{1}{2} {}^2D_{i,w}^2 \tau_{\delta,i}^{10} \tau_{\delta,\gamma,w}^0 \tau_{\delta,\gamma,w}^4 \quad (4r_D r_T^2 N_o) \quad (4669)$$

Raw expression

$${}^2R_{i,\epsilon}^2 \leftarrow - \sum_{\gamma \in A} \sum_{j \in O} \sum_{k \in O} \sum_{l \in O} \sum_{a \in V} \sum_{b \in V} \sum_{c \in V} \sum_{d \in V} {}^1T_{c,i} \\ {}^1T_{d,k} Y_{j,\gamma}^{1,*} Z_{a,\epsilon}^{*,\gamma} Y_{b,\gamma}^{3,*} Y_{j,\gamma}^{4,*} {}^2D_{a,i,b,j} {}^2T_{a,l,b,j} V_{k,d,l,c} \quad (4657)$$

Raw expression

$${}^2R_{i,\epsilon}^2 \leftarrow - \sum_{\gamma \in A} \sum_{j \in O} \sum_{k \in O} \sum_{l \in O} \sum_{a \in V} \sum_{b \in V} \sum_{c \in V} \sum_{d \in V} {}^1T_{c,i} \\ {}^1T_{d,k} Y_{j,\gamma}^{1,*} Z_{a,\epsilon}^{*,\gamma} Y_{b,\gamma}^{3,*} Y_{j,\gamma}^{4,*} {}^2D_{a,i,b,j} {}^2T_{b,j,a,l} V_{k,d,l,c} \quad (4670)$$

Factorized expression

$$\tau_{\gamma,\delta,w}^0 = \sum_{a \in V} {}^2D_{a,w}^1 Y_{a,\gamma}^1 Y_{a,\delta}^{1,*} \quad (3r_D r_T^2 N_v) \quad (4658)$$

$$\tau_{\gamma,\delta,w}^0 = \sum_{a \in V} {}^2D_{a,w}^3 Y_{a,\gamma}^1 Y_{a,\delta}^{3,*} \quad (3r_D r_T^2 N_v) \quad (4671)$$

$$\tau_{\gamma,\delta,w}^1 = \sum_{a \in V} {}^2D_{a,w}^3 Y_{a,\gamma}^3 Y_{a,\delta}^{3,*} \quad (3r_D r_T^2 N_v) \quad (4659)$$

$$\tau_{\gamma,\delta,w}^1 = \sum_{i \in O} {}^2D_{i,w}^4 Y_{i,\gamma}^2 Y_{i,\delta}^{4,*} \quad (3r_D r_T^2 N_o) \quad (4672)$$

$$\tau_{\gamma,\delta,w}^2 = \sum_{i \in O} {}^2D_{i,w}^4 Y_{i,\gamma}^4 Y_{i,\delta}^{4,*} \quad (3r_D r_T^2 N_o) \quad (4660)$$

$$\tau_{\gamma,\delta,w}^2 = \sum_{\epsilon \in A} Z_{\delta,\epsilon}^* \tau_{\gamma,\epsilon,w}^0 \tau_{\gamma,\epsilon,w}^1 \quad (3r_D r_T^3) \quad (4673)$$

$$\tau_{\gamma,\delta,w}^3 = \sum_{\epsilon \in A} Z_{\delta,\epsilon}^* \tau_{\gamma,\epsilon,w}^1 \tau_{\gamma,\epsilon,w}^2 \quad (3r_D r_T^3) \quad (4661)$$

$$\tau_{\gamma,\delta,w}^3 = \sum_{\epsilon \in A} Z_{\epsilon,\gamma} \tau_{\epsilon,\delta,w}^2 \quad (2r_D r_T^3) \quad (4674)$$

$$\tau_{\gamma,\delta,w}^4 = \sum_{\epsilon \in A} Z_{\gamma,\epsilon} \tau_{\epsilon,\delta,w}^3 \quad (2r_D r_T^3) \quad (4662)$$

$$\tau_{\gamma,\delta,w}^4 = \sum_{a \in V} {}^2D_{a,w}^1 Y_{a,\gamma}^3 Y_{a,\delta}^{1,*} \quad (3r_D r_T^2 N_v) \quad (4675)$$

$$\tau_{\alpha,i}^5 = \sum_{a \in V} {}^1T_{a,i} W_{a,\alpha}^4 \quad (2r_V N_o N_v) \quad (4663)$$

$$\tau_{\alpha,i}^5 = \sum_{a \in V} {}^1T_{a,i} W_{a,\alpha}^4 \quad (2r_V N_o N_v) \quad (4676)$$



$$\tau^6_{\alpha,\beta} = \sum_{i \in O} W^1_{i,\alpha} \tau^5_{\beta,i} \quad (2r_V^2 N_o) \quad (4677)$$

$$\tau^6_{i,j} = \sum_{a \in V} {}^1T_{a,i} \tau^5_{j,a} \quad (2N_o^2 N_v) \quad (4690)$$

$$\tau^7_{\alpha,i} = \sum_{\beta \in B} X_{\alpha,\beta} W^3_{i,\beta} \tau^6_{\alpha,\beta} \quad (3r_V^2 N_o) \quad (4678)$$

$$\tau^7_{\gamma,i} = \sum_{j \in O} Y^4_{j,\gamma} \tau^6_{i,j} \quad (2r_T N_o^2) \quad (4691)$$

$$\tau^8_{i,a} = \sum_{\alpha \in B} W^2_{a,\alpha} \tau^7_{\alpha,i} \quad (2r_V N_o N_v) \quad (4679)$$

$$\tau^8_{\gamma,\delta,w} = \sum_{i \in O} {}^2D^4_{i,w} Y^{4,*}_{i,\delta} \tau^7_{\gamma,i} \quad (3r_D r_T^2 N_o) \quad (4692)$$

$$\tau^9_{i,j} = \sum_{a \in V} {}^1T_{a,i} \tau^8_{j,a} \quad (2N_o^2 N_v) \quad (4680)$$

$$\tau^9_{\gamma,\delta,w} = \sum_{\epsilon \in A} Z^*_{\delta,\epsilon} \tau^1_{\gamma,\epsilon,w} \tau^8_{\gamma,\epsilon,w} \quad (3r_D r_T^3) \quad (4693)$$

$$\tau^{10}_{\gamma,i} = \sum_{j \in O} Y^4_{j,\gamma} \tau^9_{i,j} \quad (2r_T N_o^2) \quad (4681)$$

$$\tau^{10}_{\gamma,\delta,w} = \sum_{\epsilon \in A} Z_{\gamma,\epsilon} \tau^9_{\epsilon,\delta,w} \quad (2r_D r_T^3) \quad (4694)$$

$${}^2R^2_{i,\gamma} \leftarrow \sum_{\delta \in A} \sum_{w \in D} \frac{1}{2} {}^2D^2_{i,w} \tau^{10}_{\delta,i} \tau^3_{\delta,\gamma,w} \tau^4_{\delta,\gamma,w} \quad (4r_D r_T^2 N_o) \quad (4682)$$

$${}^2R^2_{i,\gamma} \leftarrow \sum_{\delta \in A} \sum_{w \in D} \frac{1}{2} {}^2D^2_{i,w} Y^2_{i,\delta} \tau^0_{\delta,\gamma,w} \tau^{10}_{\delta,\gamma,w} \quad (4r_D r_T^2 N_o) \quad (4695)$$

Raw expression

$${}^2R^2_{i,\epsilon} \leftarrow - \sum_{\gamma \in A} \sum_{j \in O} \sum_{k \in O} \sum_{l \in O} \sum_{a \in V} \sum_{b \in V} \sum_{c \in V} \sum_{d \in V} {}^1T_{c,k} \\ {}^1T_{d,j} Y^{1,*}_{a,\epsilon} Z^*_{\epsilon,\gamma} Y^{3,*}_{b,\gamma} \\ Y^{4,*}_{j,\gamma} {}^2D^{a,i,b,j} {}^2T_{a,i,b,l} V_{k,c,l,d} \quad (4683)$$

Raw expression

$${}^2R^2_{i,\epsilon} \leftarrow - \sum_{\gamma \in A} \sum_{j \in O} \sum_{k \in O} \sum_{l \in O} \sum_{a \in V} \sum_{b \in V} \sum_{c \in V} \sum_{d \in V} {}^1T_{c,k} \\ {}^1T_{d,j} Y^{1,*}_{a,\epsilon} Z^*_{\epsilon,\gamma} Y^{3,*}_{b,\gamma} \\ Y^{4,*}_{j,\gamma} {}^2D^{a,i,b,j} {}^2T_{b,l,a,i} V_{k,c,l,d} \quad (4696)$$

Factorized expression

$$\tau^0_{\gamma,\delta,w} = \sum_{a \in V} {}^2D^1_{a,w} Y^1_{a,\gamma} Y^{1,*}_{a,\delta} \quad (3r_D r_T^2 N_v) \quad (4684)$$

$$\tau^0_{\gamma,\delta,w} = \sum_{a \in V} {}^2D^1_{a,w} Y^3_{a,\gamma} Y^{1,*}_{a,\delta} \quad (3r_D r_T^2 N_v) \quad (4697)$$

$$\tau^1_{\gamma,\delta,w} = \sum_{a \in V} {}^2D^3_{a,w} Y^3_{a,\gamma} Y^{3,*}_{a,\delta} \quad (3r_D r_T^2 N_v) \quad (4685)$$

$$\tau^1_{\gamma,\delta,w} = \sum_{a \in V} {}^2D^3_{a,w} Y^1_{a,\gamma} Y^{3,*}_{a,\delta} \quad (3r_D r_T^2 N_v) \quad (4698)$$

$$\tau^2_{\alpha,i} = \sum_{a \in V} {}^1T_{a,i} W^4_{a,\alpha} \quad (2r_V N_o N_v) \quad (4686)$$

$$\tau^2_{\alpha,i} = \sum_{a \in V} {}^1T_{a,i} W^4_{a,\alpha} \quad (2r_V N_o N_v) \quad (4699)$$

$$\tau^3_{\alpha,\beta} = \sum_{i \in O} W^1_{i,\alpha} \tau^2_{\beta,i} \quad (2r_V^2 N_o) \quad (4687)$$

$$\tau^3_{\alpha,\beta} = \sum_{i \in O} W^1_{i,\alpha} \tau^2_{\beta,i} \quad (2r_V^2 N_o) \quad (4700)$$

$$\tau^4_{\alpha,i} = \sum_{\beta \in B} X_{\alpha,\beta} W^3_{i,\beta} \tau^3_{\alpha,\beta} \quad (3r_V^2 N_o) \quad (4688)$$

$$\tau^4_{\alpha,i} = \sum_{\beta \in B} X_{\alpha,\beta} W^3_{i,\beta} \tau^3_{\alpha,\beta} \quad (3r_V^2 N_o) \quad (4701)$$

$$\tau^5_{i,a} = \sum_{\alpha \in B} W^2_{a,\alpha} \tau^4_{\alpha,i} \quad (2r_V N_o N_v) \quad (4689)$$

$$\tau^5_{i,a} = \sum_{\alpha \in B} W^2_{a,\alpha} \tau^4_{\alpha,i} \quad (2r_V N_o N_v) \quad (4702)$$

$$\tau^6_{i,j} = \sum_{a \in V} {}^1T_{a,i} \tau^5_{j,a} \quad (2N_o^2 N_v) \quad (4703)$$

$$\tau^5_{\gamma,\alpha} = \sum_{i \in O} W^3_{i,\alpha} Y^4_{i,\gamma} \quad (2r_T r_V N_o) \quad (4715)$$

$$\tau^7_{\gamma,i} = \sum_{j \in O} Y^2_{j,\gamma} \tau^6_{i,j} \quad (2r_T N_o^2) \quad (4704)$$

$$\tau^6_{\gamma,\alpha} = \sum_{\beta \in B} X_{\alpha,\beta} \tau^4_{\gamma,\beta} \tau^5_{\gamma,\beta} \quad (3r_T r_V^2) \quad (4716)$$

$$\tau^8_{\gamma,\delta,w} = \sum_{i \in O} {}^2D^4_{i,w} Y^{4,*}_{i,\delta} \tau^7_{\gamma,i} \quad (3r_D r_T^2 N_o) \quad (4705)$$

$$\tau^7_{\gamma,\alpha} = \sum_{a \in V} W^2_{a,\alpha} Y^3_{a,\gamma} \quad (2r_T r_V N_v) \quad (4717)$$

$$\tau^9_{\gamma,\delta,w} = \sum_{\epsilon \in A} Z^*_{\delta,\epsilon} \tau^1_{\gamma,\epsilon,w} \tau^8_{\gamma,\epsilon,w} \quad (3r_D r_T^3) \quad (4706)$$

$$\tau^8_{\gamma,\alpha} = \sum_{i \in O} W^1_{i,\alpha} Y^4_{i,\gamma} \quad (2r_T r_V N_o) \quad (4718)$$

$$\tau^{10}_{\gamma,\delta,w} = \sum_{\epsilon \in A} Z_{\epsilon,\gamma} \tau^9_{\epsilon,\delta,w} \quad (2r_D r_T^3) \quad (4707)$$

$$\tau^9_{\gamma,\delta} = \sum_{\alpha \in B} \tau^6_{\delta,\alpha} \tau^7_{\gamma,\alpha} \tau^8_{\gamma,\alpha} \quad (3r_T^2 r_V) \quad (4719)$$

$${}^2R^2_{i,\gamma} \leftarrow \sum_{\delta \in A} \sum_{w \in D} \frac{1}{2} {}^2D^2_{i,w} Y^4_{i,\delta} \tau^0_{\delta,\gamma,w} \tau^{10}_{\delta,\gamma,w} \quad (4r_D r_T^2 N_o) \quad (4708)$$

$$\tau^{10}_{\gamma,\delta} = \sum_{\epsilon \in A} Z_{\gamma,\epsilon} \tau^9_{\delta,\epsilon} \quad (2r_T^3) \quad (4720)$$

$$\tau^{11}_{\gamma,\delta} = \sum_{\epsilon \in A} Z_{\gamma,\epsilon} \tau^{10}_{\delta,\epsilon} \quad (2r_T^3) \quad (4721)$$

### I. Contributions from $(H^2 T^2 T)_c$

Raw expression

$${}^2R^2_{i,\epsilon} \leftarrow \sum_{\gamma \in A} \sum_{j \in O} \sum_{k \in O} \sum_{l \in O} \sum_{a \in V} \sum_{b \in V} \sum_{c \in V} \sum_{d \in V} Y^{1,*}_{a,\epsilon} Z^*_{\epsilon,\gamma} Y^{3,*}_{b,\gamma} Y^{4,*}_{j,\gamma} {}^2D^{a,i,b,j} {}^2T_{a,i,c,k} {}^2T_{b,j,d,l} V_{k,c,l,d} \quad (4709)$$

$$\tau^{12}_{\gamma,\delta,w} = \sum_{\epsilon \in A} \tau^{11}_{\gamma,\epsilon} \tau^3_{\epsilon,\delta,w} \quad (2r_D r_T^3) \quad (4722)$$

$${}^2R^2_{i,\gamma} \leftarrow \sum_{\delta \in A} \sum_{w \in D} {}^2D^2_{i,w} Y^2_{i,\delta} \tau^0_{\delta,\gamma,w} \tau^{12}_{\delta,\gamma,w} \quad (4r_D r_T^2 N_o) \quad (4723)$$

Factorized expression

$$\tau^0_{\gamma,\delta,w} = \sum_{a \in V} {}^2D^1_{a,w} Y^1_{a,\gamma} Y^{1,*}_{a,\delta} \quad (3r_D r_T^2 N_v) \quad (4710)$$

Raw expression

$${}^2R^2_{i,\epsilon} \leftarrow \sum_{\gamma \in A} \sum_{j \in O} \sum_{k \in O} \sum_{l \in O} \sum_{a \in V} \sum_{b \in V} \sum_{c \in V} \sum_{d \in V} Y^{1,*}_{a,\epsilon} Z^*_{\epsilon,\gamma} Y^{3,*}_{b,\gamma} Y^{4,*}_{j,\gamma} {}^2D^{a,i,b,j} {}^2T_{a,i,c,k} {}^2T_{d,l,b,j} V_{k,c,l,d} \quad (4724)$$

$$\tau^1_{\gamma,\delta,w} = \sum_{a \in V} {}^2D^3_{a,w} Y^1_{a,\gamma} Y^{3,*}_{a,\delta} \quad (3r_D r_T^2 N_v) \quad (4711)$$

Factorized expression

$$\tau^2_{\gamma,\delta,w} = \sum_{i \in O} {}^2D^4_{i,w} Y^2_{i,\gamma} Y^{4,*}_{i,\delta} \quad (3r_D r_T^2 N_o) \quad (4712)$$

$$\tau^0_{\gamma,\delta,w} = \sum_{a \in V} {}^2D^1_{a,w} Y^1_{a,\gamma} Y^{1,*}_{a,\delta} \quad (3r_D r_T^2 N_v) \quad (4725)$$

$$\tau^3_{\gamma,\delta,w} = \sum_{\epsilon \in A} Z^*_{\delta,\epsilon} \tau^1_{\gamma,\epsilon,w} \tau^2_{\gamma,\epsilon,w} \quad (3r_D r_T^3) \quad (4713)$$

$$\tau^1_{\gamma,\delta,w} = \sum_{a \in V} {}^2D^3_{a,w} Y^3_{a,\gamma} Y^{3,*}_{a,\delta} \quad (3r_D r_T^2 N_v) \quad (4726)$$

$$\tau^4_{\gamma,\alpha} = \sum_{a \in V} W^4_{a,\alpha} Y^3_{a,\gamma} \quad (2r_T r_V N_v) \quad (4714)$$

$$\tau^2_{\gamma,\delta,w} = \sum_{i \in O} {}^2D^4_{i,w} Y^4_{i,\gamma} Y^{4,*}_{i,\delta} \quad (3r_D r_T^2 N_o) \quad (4727)$$

$$\tau^3_{\gamma,\delta,w} = \sum_{\epsilon \in A} Z^*_{\delta,\epsilon} \tau^1_{\gamma,\epsilon,w} \tau^2_{\gamma,\epsilon,w} \quad (3r_D r_T^3) \quad (4728)$$

$$\tau^1_{\gamma,\delta,w} = \sum_{a \in V} {}^2D^3_{a,w} Y^1_{a,\gamma} Y^{3,*}_{a,\delta} \quad (3r_D r_T^2 N_v) \quad (4741)$$

$$\tau^4_{\gamma,\alpha} = \sum_{a \in V} W^2_{a,\alpha} Y^3_{a,\gamma} \quad (2r_T r_V N_v) \quad (4729)$$

$$\tau^2_{\gamma,\delta,w} = \sum_{i \in O} {}^2D^4_{i,w} Y^2_{i,\gamma} Y^{4,*}_{i,\delta} \quad (3r_D r_T^2 N_o) \quad (4742)$$

$$\tau^5_{\gamma,\alpha} = \sum_{i \in O} W^1_{i,\alpha} Y^4_{i,\gamma} \quad (2r_T r_V N_o) \quad (4730)$$

$$\tau^3_{\gamma,\delta,w} = \sum_{\epsilon \in A} Z^*_{\delta,\epsilon} \tau^1_{\gamma,\epsilon,w} \tau^2_{\gamma,\epsilon,w} \quad (3r_D r_T^3) \quad (4743)$$

$$\tau^6_{\gamma,\alpha} = \sum_{a \in V} W^4_{a,\alpha} Y^1_{a,\gamma} \quad (2r_T r_V N_v) \quad (4731)$$

$$\tau^4_{\gamma,\alpha} = \sum_{a \in V} W^4_{a,\alpha} Y^3_{a,\gamma} \quad (2r_T r_V N_v) \quad (4744)$$

$$\tau^7_{\gamma,\alpha} = \sum_{i \in O} W^3_{i,\alpha} Y^2_{i,\gamma} \quad (2r_T r_V N_o) \quad (4732)$$

$$\tau^5_{\gamma,\alpha} = \sum_{i \in O} W^3_{i,\alpha} Y^4_{i,\gamma} \quad (2r_T r_V N_o) \quad (4745)$$

$$\tau^8_{\gamma,\alpha} = \sum_{\beta \in B} X_{\alpha,\beta} \tau^6_{\gamma,\beta} \tau^7_{\gamma,\beta} \quad (3r_T r_V^2) \quad (4733)$$

$$\tau^6_{\gamma,\alpha} = \sum_{\beta \in B} X_{\alpha,\beta} \tau^4_{\gamma,\beta} \tau^5_{\gamma,\beta} \quad (3r_T r_V^2) \quad (4746)$$

$$\tau^9_{\gamma,\delta} = \sum_{\alpha \in B} \tau^4_{\delta,\alpha} \tau^5_{\delta,\alpha} \tau^8_{\gamma,\alpha} \quad (3r_T^2 r_V) \quad (4734)$$

$$\tau^7_{\gamma,\alpha} = \sum_{a \in V} W^2_{a,\alpha} Y^1_{a,\gamma} \quad (2r_T r_V N_v) \quad (4747)$$

$$\tau^{10}_{\gamma,\delta} = \sum_{\epsilon \in A} Z_{\delta,\epsilon} \tau^9_{\gamma,\epsilon} \quad (2r_T^3) \quad (4735)$$

$$\tau^8_{\gamma,\alpha} = \sum_{i \in O} W^1_{i,\alpha} Y^2_{i,\gamma} \quad (2r_T r_V N_o) \quad (4748)$$

$$\tau^{11}_{\gamma,\delta} = \sum_{\epsilon \in A} Z_{\epsilon,\delta} \tau^{10}_{\epsilon,\gamma} \quad (2r_T^3) \quad (4736)$$

$$\tau^9_{\gamma,\delta} = \sum_{\alpha \in B} \tau^6_{\delta,\alpha} \tau^7_{\gamma,\alpha} \tau^8_{\gamma,\alpha} \quad (3r_T^2 r_V) \quad (4749)$$

$$\tau^{12}_{\gamma,\delta,w} = \sum_{\epsilon \in A} \tau^{11}_{\gamma,\epsilon} \tau^3_{\epsilon,\delta,w} \quad (2r_D r_T^3) \quad (4737)$$

$$\tau^{10}_{\gamma,\delta} = \sum_{\epsilon \in A} Z_{\delta,\epsilon} \tau^9_{\gamma,\epsilon} \quad (2r_T^3) \quad (4750)$$

$${}^2R^2_{i,\gamma} \leftarrow \sum_{\delta \in A} \sum_{w \in D} {}^2D^2_{i,w} Y^2_{i,\delta} \tau^0_{\delta,\gamma,w} \tau^{12}_{\delta,\gamma,w} \quad (4r_D r_T^2 N_o) \quad (4738)$$

$$\tau^{11}_{\gamma,\delta} = \sum_{\epsilon \in A} Z_{\epsilon,\delta} \tau^{10}_{\epsilon,\gamma} \quad (2r_T^3) \quad (4751)$$

$$\tau^{12}_{\gamma,\delta,w} = \sum_{\epsilon \in A} \tau^{11}_{\epsilon,\gamma} \tau^3_{\epsilon,\delta,w} \quad (2r_D r_T^3) \quad (4752)$$

Raw expression

$${}^2R^2_{i,\epsilon} \leftarrow \sum_{\gamma \in A} \sum_{j \in O} \sum_{k \in O} \sum_{l \in O} \sum_{a \in V} \sum_{b \in V} \sum_{c \in V} \sum_{d \in V} Y^{1,*}_{a,\epsilon} Z^*_{\epsilon,\gamma} Y^{3,*}_{b,\gamma} Y^{4,*}_{j,\gamma} {}^2D^{a,i,b,j} {}^2T_{b,j,d,l} {}^2T_{c,k,a,i} V_{k,c,l,d} \quad (4739)$$

$${}^2R^2_{i,\gamma} \leftarrow \sum_{\delta \in A} \sum_{w \in D} {}^2D^2_{i,w} Y^4_{i,\delta} \tau^0_{\delta,\gamma,w} \tau^{12}_{\delta,\gamma,w} \quad (4r_D r_T^2 N_o) \quad (4753)$$

Raw expression

Factorized expression

$$\tau^0_{\gamma,\delta,w} = \sum_{a \in V} {}^2D^1_{a,w} Y^3_{a,\gamma} Y^{1,*}_{a,\delta} \quad (3r_D r_T^2 N_v) \quad (4740)$$

$${}^2R^2_{i,\epsilon} \leftarrow \sum_{\gamma \in A} \sum_{j \in O} \sum_{k \in O} \sum_{l \in O} \sum_{a \in V} \sum_{b \in V} \sum_{c \in V} \sum_{d \in V} Y^{1,*}_{a,\epsilon} Z^*_{\epsilon,\gamma} Y^{3,*}_{b,\gamma} Y^{4,*}_{j,\gamma} {}^2D^{a,i,b,j} {}^2T_{c,k,a,i} {}^2T_{d,l,b,j} V_{k,c,l,d} \quad (4754)$$

Factorized expression

$$\tau_{\gamma,\delta,w}^0 = \sum_{a \in V} {}^2D_{a,w}^1 Y_{a,\gamma}^3 Y_{a,\delta}^{1,*} \quad (3r_D r_T^2 N_v) \quad (4755)$$

$$\tau_{\gamma,\delta,w}^1 = \sum_{a \in V} {}^2D_{a,w}^3 Y_{a,\gamma}^3 Y_{a,\delta}^{3,*} \quad (3r_D r_T^2 N_v) \quad (4756)$$

$$\tau_{\gamma,\delta,w}^2 = \sum_{i \in O} {}^2D_{i,w}^4 Y_{i,\gamma}^4 Y_{i,\delta}^{4,*} \quad (3r_D r_T^2 N_o) \quad (4757)$$

$$\tau_{\gamma,\delta,w}^3 = \sum_{\epsilon \in A} Z_{\delta,\epsilon}^* \tau_{\gamma,\epsilon,w}^1 \tau_{\gamma,\epsilon,w}^2 \quad (3r_D r_T^3) \quad (4758)$$

$$\tau_{\gamma,\alpha}^4 = \sum_{a \in V} W_{a,\alpha}^4 Y_{a,\gamma}^1 \quad (2r_T r_V N_v) \quad (4759)$$

$$\tau_{\gamma,\alpha}^5 = \sum_{i \in O} W_{i,\alpha}^3 Y_{i,\gamma}^2 \quad (2r_T r_V N_o) \quad (4760)$$

$$\tau_{\gamma,\alpha}^6 = \sum_{\beta \in B} X_{\alpha,\beta} \tau_{\gamma,\beta}^4 \tau_{\gamma,\beta}^5 \quad (3r_T r_V^2) \quad (4761)$$

$$\tau_{\gamma,\alpha}^7 = \sum_{a \in V} W_{a,\alpha}^2 Y_{a,\gamma}^1 \quad (2r_T r_V N_v) \quad (4762)$$

$$\tau_{\gamma,\alpha}^8 = \sum_{i \in O} W_{i,\alpha}^1 Y_{i,\gamma}^2 \quad (2r_T r_V N_o) \quad (4763)$$

$$\tau_{\gamma,\delta}^9 = \sum_{\alpha \in B} \tau_{\delta,\alpha}^6 \tau_{\gamma,\alpha}^7 \tau_{\gamma,\alpha}^8 \quad (3r_T^2 r_V) \quad (4764)$$

$$\tau_{\gamma,\delta}^{10} = \sum_{\epsilon \in A} Z_{\epsilon,\delta} \tau_{\gamma,\epsilon}^9 \quad (2r_T^3) \quad (4765)$$

$$\tau_{\gamma,\delta}^{11} = \sum_{\epsilon \in A} Z_{\epsilon,\gamma} \tau_{\epsilon,\delta}^{10} \quad (2r_T^3) \quad (4766)$$

$$\tau_{\gamma,\delta,w}^{12} = \sum_{\epsilon \in A} \tau_{\gamma,\epsilon}^{11} \tau_{\epsilon,\delta,w}^3 \quad (2r_D r_T^3) \quad (4767)$$

$${}^2R_{i,\gamma}^2 \leftarrow \sum_{\delta \in A} \sum_{w \in D} {}^2D_{i,w}^2 Y_{i,\delta}^4 \tau_{\delta,\gamma,w}^0 \tau_{\delta,\gamma,w}^{12} \quad (4r_D r_T^2 N_o) \quad (4768)$$

Raw expression

$${}^2R_{i,\epsilon}^2 \leftarrow - \sum_{\gamma \in A} \sum_{j \in O} \sum_{k \in O} \sum_{l \in O} \sum_{a \in V} \sum_{b \in V} \sum_{c \in V} \sum_{d \in V} \frac{1}{2} \quad (4769)$$

$$Y_{a,\epsilon}^{1,*} Z_{\epsilon,\gamma}^* Y_{b,\gamma}^{3,*} Y_{j,\gamma}^{4,*} {}^2D_{a,i,b,j} {}^2T_{a,i,b,k} {}^2T_{c,j,d,l} V_{k,c,l,d}$$

Factorized expression

$$\tau_{\gamma,\delta,w}^0 = \sum_{a \in V} {}^2D_{a,w}^1 Y_{a,\gamma}^1 Y_{a,\delta}^{1,*} \quad (3r_D r_T^2 N_v) \quad (4770)$$

$$\tau_{\gamma,\delta,w}^1 = \sum_{a \in V} {}^2D_{a,w}^3 Y_{a,\gamma}^1 Y_{a,\delta}^{3,*} \quad (3r_D r_T^2 N_v) \quad (4771)$$

$$\tau_{\gamma,\delta,w}^2 = \sum_{i \in O} {}^2D_{i,w}^4 Y_{i,\gamma}^2 Y_{i,\delta}^{4,*} \quad (3r_D r_T^2 N_o) \quad (4772)$$

$$\tau_{\gamma,\delta,w}^3 = \sum_{\epsilon \in A} Z_{\delta,\epsilon}^* \tau_{\gamma,\epsilon,w}^1 \tau_{\gamma,\epsilon,w}^2 \quad (3r_D r_T^3) \quad (4773)$$

$$\tau_{\gamma,\alpha}^4 = \sum_{a \in V} W_{a,\alpha}^2 Y_{a,\gamma}^3 \quad (2r_T r_V N_v) \quad (4774)$$

$$\tau_{\gamma,\alpha,i}^5 = \sum_{\beta \in B} W_{i,\beta}^1 X_{\beta,\alpha} \tau_{\gamma,\beta}^4 \quad (3r_T r_V^2 N_o) \quad (4775)$$

$$\tau_{\gamma,\alpha}^6 = \sum_{i \in O} W_{i,\alpha}^3 Y_{i,\gamma}^4 \quad (2r_T r_V N_o) \quad (4776)$$

$$\tau_{\gamma,\alpha}^7 = \sum_{a \in V} W_{a,\alpha}^4 Y_{a,\gamma}^3 \quad (2r_T r_V N_v) \quad (4777)$$

$$\tau_{\gamma,\delta,i}^8 = \sum_{\alpha \in B} \tau_{\gamma,\alpha}^6 \tau_{\delta,\alpha}^7 \tau_{\gamma,\alpha,i}^5 \quad (3r_T^2 r_V N_o) \quad (4778)$$

$$\tau_{\gamma,\delta}^9 = \sum_{i \in O} Y_{i,\delta}^4 \tau_{\gamma,\delta,i}^8 \quad (2r_T^2 N_o) \quad (4779)$$

$$\tau_{\gamma,\delta}^{10} = \sum_{\epsilon \in A} Z_{\gamma,\epsilon} \tau_{\delta,\epsilon}^9 \quad (2r_T^3) \quad (4780)$$

$$\tau_{\gamma,\delta}^{11} = \sum_{\epsilon \in A} Z_{\gamma,\epsilon} \tau_{\delta,\epsilon}^{10} \quad (2r_T^3) \quad (4781)$$

$$\tau_{\gamma,\delta,w}^{12} = \sum_{\epsilon \in A} \tau_{\epsilon,\gamma}^{11} \tau_{\epsilon,\delta,w}^3 \quad (2r_D r_T^3) \quad (4782)$$

$${}^2R^2_{i,\gamma} \leftarrow - \sum_{\delta \in A} \sum_{w \in D} \frac{1}{2} {}^2D^2_{i,w} Y^2_{i,\delta} \tau^0_{\delta,\gamma,w} \tau^{12}_{\delta,\gamma,w} \quad (4r_D r_T^2 N_o) \tau^{11}_{\gamma,\delta,w} = \sum_{\epsilon \in A} Z^*_{\delta,\epsilon} \tau^{10}_{\gamma,\epsilon,w} \tau^9_{\gamma,\epsilon,w} \quad (3r_D r_T^3) \quad (4796)$$

$$(4783)$$

Raw expression

$$\tau^{12}_{\gamma,\delta,w} = \sum_{\epsilon \in A} Z_{\gamma,\epsilon} \tau^{11}_{\epsilon,\delta,w} \quad (2r_D r_T^3) \quad (4797)$$

$${}^2R^2_{i,\epsilon} \leftarrow - \sum_{\gamma \in A} \sum_{j \in O} \sum_{k \in O} \sum_{l \in O} \sum_{a \in V} \sum_{b \in V} \sum_{c \in V} \sum_{d \in V} \frac{1}{2} \quad (4784)$$

$$Y^{1,*}_{a,\epsilon} \quad Z^*_{\epsilon,\gamma} \quad Y^{3,*}_{b,\gamma} \quad Y^{4,*}_{j,\gamma}$$

$${}^2D^{a,i,b,j} \quad {}^2T_{a,i,b,k} \quad {}^2T_{c,l,d,j} \quad V_{k,d,l,c}$$

$${}^2R^2_{i,\gamma} \leftarrow - \sum_{\delta \in A} \sum_{w \in D} \frac{1}{2} {}^2D^2_{i,w} Y^2_{i,\delta} \tau^0_{\delta,\gamma,w} \tau^{12}_{\delta,\gamma,w} \quad (4r_D r_T^2 N_o) \quad (4798)$$

Factorized expression

Raw expression

$$\tau^0_{\gamma,\delta,w} = \sum_{a \in V} {}^2D^1_{a,w} Y^1_{a,\gamma} Y^{1,*}_{a,\delta} \quad (3r_D r_T^2 N_v) \quad (4785)$$

$${}^2R^2_{i,\epsilon} \leftarrow - \sum_{\gamma \in A} \sum_{j \in O} \sum_{k \in O} \sum_{l \in O} \sum_{a \in V} \sum_{b \in V} \sum_{c \in V} \sum_{d \in V} \frac{1}{2} \quad (4799)$$

$$Y^{1,*}_{a,\epsilon} \quad Z^*_{\epsilon,\gamma} \quad Y^{3,*}_{b,\gamma} \quad Y^{4,*}_{j,\gamma}$$

$${}^2D^{a,i,b,j} \quad {}^2T_{a,i,c,j} \quad {}^2T_{b,k,d,l} \quad V_{k,c,l,d}$$

$$\tau^1_{\gamma,\alpha} = \sum_{i \in O} W^1_{i,\alpha} Y^2_{i,\gamma} \quad (2r_T r_V N_o) \quad (4786)$$

Factorized expression

$$\tau^2_{\gamma,\alpha} = \sum_{a \in V} W^4_{a,\alpha} Y^3_{a,\gamma} \quad (2r_T r_V N_v) \quad (4787)$$

$$\tau^0_{\gamma,\delta,w} = \sum_{a \in V} {}^2D^1_{a,w} Y^1_{a,\gamma} Y^{1,*}_{a,\delta} \quad (3r_D r_T^2 N_v) \quad (4800)$$

$$\tau^3_{\gamma,\alpha} = \sum_{i \in O} W^3_{i,\alpha} Y^4_{i,\gamma} \quad (2r_T r_V N_o) \quad (4788)$$

$$\tau^1_{\gamma,\delta,w} = \sum_{a \in V} {}^2D^3_{a,w} Y^1_{a,\gamma} Y^{3,*}_{a,\delta} \quad (3r_D r_T^2 N_v) \quad (4801)$$

$$\tau^4_{\gamma,\alpha} = \sum_{\beta \in B} X_{\alpha,\beta} \tau^2_{\gamma,\beta} \tau^3_{\gamma,\beta} \quad (3r_T r_V^2) \quad (4789)$$

$$\tau^2_{\gamma,\alpha} = \sum_{a \in V} W^2_{a,\alpha} Y^3_{a,\gamma} \quad (2r_T r_V N_v) \quad (4802)$$

$$\tau^5_{\gamma,\alpha} = \sum_{\delta \in A} Z_{\gamma,\delta} \tau^4_{\delta,\alpha} \quad (2r_T^2 r_V) \quad (4790)$$

$$\tau^3_{\gamma,\alpha} = \sum_{i \in O} W^1_{i,\alpha} Y^4_{i,\gamma} \quad (2r_T r_V N_o) \quad (4803)$$

$$\tau^6_{\gamma,a} = \sum_{\alpha \in B} W^2_{a,\alpha} \tau^1_{\gamma,\alpha} \tau^5_{\gamma,\alpha} \quad (3r_T r_V N_v) \quad (4791)$$

$$\tau^4_{\gamma,\alpha} = \sum_{\beta \in B} X_{\beta,\alpha} \tau^2_{\gamma,\beta} \tau^3_{\gamma,\beta} \quad (3r_T r_V^2) \quad (4804)$$

$$\tau^7_{a,b} = \sum_{\gamma \in A} Y^1_{b,\gamma} \tau^6_{\gamma,a} \quad (2r_T N_v^2) \quad (4792)$$

$$\tau^5_{\gamma,\alpha} = \sum_{\delta \in A} Z_{\gamma,\delta} \tau^4_{\delta,\alpha} \quad (2r_T^2 r_V) \quad (4805)$$

$$\tau^8_{\gamma,a} = \sum_{b \in V} Y^3_{b,\gamma} \tau^7_{b,a} \quad (2r_T N_v^2) \quad (4793)$$

$$\tau^6_{\gamma,\alpha} = \sum_{a \in V} W^4_{a,\alpha} Y^3_{a,\gamma} \quad (2r_T r_V N_v) \quad (4806)$$

$$\tau^9_{\gamma,\delta,w} = \sum_{a \in V} {}^2D^3_{a,w} Y^{3,*}_{a,\delta} \tau^8_{\gamma,a} \quad (3r_D r_T^2 N_v) \quad (4794)$$

$$\tau^7_{\gamma,\delta,i} = \sum_{\alpha \in B} W^3_{i,\alpha} \tau^5_{\gamma,\alpha} \tau^6_{\delta,\alpha} \quad (3r_T^2 r_V N_o) \quad (4807)$$

$$\tau^{10}_{\gamma,\delta,w} = \sum_{i \in O} {}^2D^4_{i,w} Y^4_{i,\gamma} Y^{4,*}_{i,\delta} \quad (3r_D r_T^2 N_o) \quad (4795)$$

$$\tau^8_{\gamma,\delta,\epsilon} = \sum_{i \in O} Y^2_{i,\gamma} \tau^7_{\delta,\epsilon,i} \quad (2r_T^3 N_o) \quad (4808)$$

$$\tau_{\gamma,\delta,i}^9 = \sum_{\epsilon \in A} Z_{\gamma,\epsilon} Y_{i,\epsilon}^4 \tau_{\gamma,\delta,\epsilon}^8 \quad (3r_T^3 N_o) \quad (4809)$$

$$\tau_{i,j}^8 = \sum_{\gamma \in A} Y_{j,\gamma}^2 \tau_{\gamma,i}^7 \quad (2r_T N_o^2) \quad (4822)$$

$$\tau_{\gamma,\delta,w}^{10} = \sum_{\epsilon \in A} \sum_{i \in O} {}^2D_{i,w}^4 Y_{i,\delta}^{4,*} \tau_{\epsilon,\delta,w}^1 \tau_{\epsilon,\gamma,i}^9 \quad (4r_D r_T^3 N_o) \quad (4810)$$

$$\tau_{\gamma,i}^9 = \sum_{j \in O} Y_{j,\gamma}^4 \tau_{j,i}^8 \quad (2r_T N_o^2) \quad (4823)$$

$$\tau_{\gamma,\delta,w}^{11} = \sum_{\epsilon \in A} Z_{\delta,\epsilon}^* \tau_{\gamma,\epsilon,w}^{10} \quad (2r_D r_T^3) \quad (4811)$$

$$\tau_{\gamma,\delta,w}^{10} = \sum_{i \in O} {}^2D_{i,w}^4 Y_{i,\delta}^{4,*} \tau_{\gamma,i}^9 \quad (3r_D r_T^2 N_o) \quad (4824)$$

$${}^2R_{i,\gamma}^2 \leftarrow - \sum_{\delta \in A} \sum_{w \in D} \frac{1}{2} {}^2D_{i,w}^2 Y_{i,\delta}^{2,*} \tau_{\delta,\gamma,w}^0 \tau_{\delta,\gamma,w}^{11} \quad (4r_D r_T^2 N_o) \quad (4812)$$

$$\tau_{\gamma,\delta,w}^{11} = \sum_{\epsilon \in A} Z_{\delta,\epsilon}^* \tau_{\gamma,\epsilon,w}^1 \tau_{\gamma,\epsilon,w}^{10} \quad (3r_D r_T^3) \quad (4825)$$

Raw expression

$$\tau_{\gamma,\delta,w}^{12} = \sum_{\epsilon \in A} Z_{\gamma,\epsilon} \tau_{\epsilon,\delta,w}^{11} \quad (2r_D r_T^3) \quad (4826)$$

$${}^2R_{i,\epsilon}^2 \leftarrow - \sum_{\gamma \in A} \sum_{j \in O} \sum_{k \in O} \sum_{l \in O} \sum_{a \in V} \sum_{b \in V} \sum_{c \in V} \sum_{d \in V} \frac{1}{2} \quad (4813)$$

$$\begin{aligned} & Y_{a,\epsilon}^{1,*} Z_{\epsilon,\gamma}^* Y_{b,\gamma}^{3,*} Y_{j,\gamma}^{4,*} \\ & {}^2D_{a,i,b,j} {}^2T_{a,i,c,j} {}^2T_{d,k,b,l} V_{k,d,l,c} \end{aligned}$$

$${}^2R_{i,\gamma}^2 \leftarrow - \sum_{\delta \in A} \sum_{w \in D} \frac{1}{2} {}^2D_{i,w}^2 Y_{i,\delta}^2 \tau_{\delta,\gamma,w}^0 \tau_{\delta,\gamma,w}^{12} \quad (4r_D r_T^2 N_o) \quad (4827)$$

Factorized expression

Raw expression

$$\tau_{\gamma,\delta,w}^0 = \sum_{a \in V} {}^2D_{a,w}^1 Y_{a,\gamma}^1 Y_{a,\delta}^{1,*} \quad (3r_D r_T^2 N_v) \quad (4814)$$

$${}^2R_{i,\epsilon}^2 \leftarrow - \sum_{\gamma \in A} \sum_{j \in O} \sum_{k \in O} \sum_{l \in O} \sum_{a \in V} \sum_{b \in V} \sum_{c \in V} \sum_{d \in V} \frac{1}{2} \quad (4828)$$

$$\begin{aligned} & Y_{a,\epsilon}^{1,*} Z_{\epsilon,\gamma}^* Y_{b,\gamma}^{3,*} Y_{j,\gamma}^{4,*} \\ & {}^2D_{a,i,b,j} {}^2T_{a,i,c,k} {}^2T_{b,j,d,l} V_{k,d,l,c} \end{aligned}$$

$$\tau_{\gamma,\delta,w}^1 = \sum_{a \in V} {}^2D_{a,w}^3 Y_{a,\gamma}^3 Y_{a,\delta}^{3,*} \quad (3r_D r_T^2 N_v) \quad (4815)$$

Factorized expression

$$\tau_{\gamma,\alpha}^2 = \sum_{a \in V} W_{a,\alpha}^2 Y_{a,\gamma}^1 \quad (2r_T r_V N_v) \quad (4816)$$

$$\tau_{\gamma,\delta,w}^0 = \sum_{a \in V} {}^2D_{a,w}^1 Y_{a,\gamma}^1 Y_{a,\delta}^{1,*} \quad (3r_D r_T^2 N_v) \quad (4829)$$

$$\tau_{\gamma,\alpha}^3 = \sum_{a \in V} W_{a,\alpha}^4 Y_{a,\gamma}^3 \quad (2r_T r_V N_v) \quad (4817)$$

$$\tau_{\gamma,\alpha}^1 = \sum_{a \in V} W_{a,\alpha}^2 Y_{a,\gamma}^1 \quad (2r_T r_V N_v) \quad (4830)$$

$$\tau_{\gamma,\alpha}^4 = \sum_{i \in O} W_{i,\alpha}^3 Y_{i,\gamma}^4 \quad (2r_T r_V N_o) \quad (4818)$$

$$\tau_{\gamma,\alpha}^2 = \sum_{i \in O} W_{i,\alpha}^1 Y_{i,\gamma}^2 \quad (2r_T r_V N_o) \quad (4831)$$

$$\tau_{\gamma,\alpha}^5 = \sum_{\beta \in B} X_{\alpha,\beta} \tau_{\gamma,\beta}^3 \tau_{\gamma,\beta}^4 \quad (3r_T r_V^2) \quad (4819)$$

$$\tau_{\gamma,\alpha}^3 = \sum_{\beta \in B} X_{\beta,\alpha} \tau_{\gamma,\beta}^1 \tau_{\gamma,\beta}^2 \quad (3r_T r_V^2) \quad (4832)$$

$$\tau_{\gamma,\alpha}^6 = \sum_{\delta \in A} Z_{\gamma,\delta} \tau_{\delta,\alpha}^5 \quad (2r_T^2 r_V) \quad (4820)$$

$$\tau_{\gamma,\alpha}^4 = \sum_{\delta \in A} Z_{\delta,\gamma} \tau_{\delta,\alpha}^3 \quad (2r_T^2 r_V) \quad (4833)$$

$$\tau_{\gamma,i}^7 = \sum_{\alpha \in B} W_{i,\alpha}^1 \tau_{\gamma,\alpha}^2 \tau_{\gamma,\alpha}^6 \quad (3r_T r_V N_o) \quad (4821)$$

$$\tau_{\gamma,\alpha}^5 = \sum_{i \in O} W_{i,\alpha}^3 Y_{i,\gamma}^4 \quad (2r_T r_V N_o) \quad (4834)$$

$$\tau_{\gamma,a}^6 = \sum_{\alpha \in B} W_{a,\alpha}^4 \tau_{\gamma,\alpha}^4 \tau_{\gamma,\alpha}^5 \quad (3r_T r_V N_v) \quad (4835)$$

$$\tau_{\gamma,\alpha}^4 = \sum_{a \in V} W_{a,\alpha}^2 Y_{a,\gamma}^1 \quad (2r_T r_V N_v) \quad (4848)$$

$$\tau_{\gamma,\delta}^7 = \sum_{a \in V} Y_{a,\delta}^3 \tau_{\gamma,a}^6 \quad (2r_T^2 N_v) \quad (4836)$$

$$\tau_{\gamma,\alpha,i}^5 = \sum_{\beta \in B} W_{i,\beta}^1 X_{\beta,\alpha} \tau_{\gamma,\beta}^4 \quad (3r_T r_V^2 N_o) \quad (4849)$$

$$\tau_{\gamma,a}^8 = \sum_{\delta \in A} Y_{a,\delta}^3 \tau_{\delta,\gamma}^7 \quad (2r_T^2 N_v) \quad (4837)$$

$$\tau_{\gamma,\alpha}^6 = \sum_{i \in O} W_{i,\alpha}^3 Y_{i,\gamma}^2 \quad (2r_T r_V N_o) \quad (4850)$$

$$\tau_{\gamma,\delta,w}^9 = \sum_{a \in V} {}^2D_{a,w}^3 Y_{a,\gamma}^{3,*} \tau_{\gamma,a}^8 \quad (3r_D r_T^2 N_v) \quad (4838)$$

$$\tau_{\gamma,\alpha}^7 = \sum_{a \in V} W_{a,\alpha}^4 Y_{a,\gamma}^3 \quad (2r_T r_V N_v) \quad (4851)$$

$$\tau_{\gamma,\delta,w}^{10} = \sum_{i \in O} {}^2D_{i,w}^4 Y_{i,\gamma}^4 Y_{i,\delta}^{4,*} \quad (3r_D r_T^2 N_o) \quad (4839)$$

$$\tau_{\gamma,\delta,i}^8 = \sum_{\alpha \in B} \tau_{\gamma,\alpha}^6 \tau_{\delta,\alpha}^7 \tau_{\gamma,\alpha,i}^5 \quad (3r_T^2 r_V N_o) \quad (4852)$$

$$\tau_{\gamma,\delta,w}^{11} = \sum_{\epsilon \in A} Z_{\delta,\epsilon}^* \tau_{\gamma,\epsilon,w}^{10} \tau_{\gamma,\epsilon,w}^9 \quad (3r_D r_T^3) \quad (4840)$$

$$\tau_{\gamma,\delta}^9 = \sum_{i \in O} Y_{i,\delta}^4 \tau_{\gamma,\delta,i}^8 \quad (2r_T^2 N_o) \quad (4853)$$

$$\tau_{\gamma,\delta,w}^{12} = \sum_{\epsilon \in A} Z_{\gamma,\epsilon} \tau_{\epsilon,\delta,w}^{11} \quad (2r_D r_T^3) \quad (4841)$$

$$\tau_{\gamma,\delta}^{10} = \sum_{\epsilon \in A} Z_{\delta,\epsilon} \tau_{\gamma,\epsilon}^9 \quad (2r_T^3) \quad (4854)$$

$${}^2R_{i,\gamma}^2 \leftarrow - \sum_{\delta \in A} \sum_{w \in D} \frac{1}{2} {}^2D_{i,w}^2 Y_{i,\delta}^2 \tau_{\delta,\gamma,w}^0 \tau_{\delta,\gamma,w}^{12} \quad (4r_D r_T^2 N_o) \quad (4842)$$

$$\tau_{\gamma,\delta}^{11} = \sum_{\epsilon \in A} Z_{\epsilon,\delta} \tau_{\epsilon,\gamma}^{10} \quad (2r_T^3) \quad (4855)$$

Raw expression

$$\tau_{\gamma,\delta,w}^{12} = \sum_{\epsilon \in A} \tau_{\gamma,\epsilon}^{11} \tau_{\epsilon,\delta,w}^3 \quad (2r_D r_T^3) \quad (4856)$$

$${}^2R_{i,\epsilon}^2 \leftarrow - \sum_{\gamma \in A} \sum_{j \in O} \sum_{k \in O} \sum_{l \in O} \sum_{a \in V} \sum_{b \in V} \sum_{c \in V} \sum_{d \in V} \frac{1}{2} \quad (4843)$$

$$Y_{a,\epsilon}^{1,*} Z_{\epsilon,\gamma}^* Y_{b,\gamma}^{3,*} Y_{j,\gamma}^{4,*} {}^2D_{a,i,b,j} {}^2T_{a,i,c,k} {}^2T_{b,l,d,j} V_{k,c,l,d}$$

$${}^2R_{i,\gamma}^2 \leftarrow - \sum_{\delta \in A} \sum_{w \in D} \frac{1}{2} {}^2D_{i,w}^2 Y_{i,\delta}^2 \tau_{\delta,\gamma,w}^0 \tau_{\delta,\gamma,w}^{12} \quad (4r_D r_T^2 N_o) \quad (4857)$$

Factorized expression

Raw expression

$$\tau_{\gamma,\delta,w}^0 = \sum_{a \in V} {}^2D_{a,w}^1 Y_{a,\gamma}^1 Y_{a,\delta}^{1,*} \quad (3r_D r_T^2 N_v) \quad (4844)$$

$${}^2R_{i,\epsilon}^2 \leftarrow - \sum_{\gamma \in A} \sum_{j \in O} \sum_{k \in O} \sum_{l \in O} \sum_{a \in V} \sum_{b \in V} \sum_{c \in V} \sum_{d \in V} \frac{1}{2} \quad (4858)$$

$$Y_{a,\epsilon}^{1,*} Z_{\epsilon,\gamma}^* Y_{b,\gamma}^{3,*} Y_{j,\gamma}^{4,*} {}^2D_{a,i,b,j} {}^2T_{a,i,c,k} {}^2T_{d,j,b,l} V_{k,c,l,d}$$

$$\tau_{\gamma,\delta,w}^1 = \sum_{a \in V} {}^2D_{a,w}^3 Y_{a,\gamma}^3 Y_{a,\delta}^{3,*} \quad (3r_D r_T^2 N_v) \quad (4845)$$

Factorized expression

$$\tau_{\gamma,\delta,w}^2 = \sum_{i \in O} {}^2D_{i,w}^4 Y_{i,\gamma}^4 Y_{i,\delta}^{4,*} \quad (3r_D r_T^2 N_o) \quad (4846)$$

$$\tau_{\gamma,\delta,w}^0 = \sum_{a \in V} {}^2D_{a,w}^1 Y_{a,\gamma}^1 Y_{a,\delta}^{1,*} \quad (3r_D r_T^2 N_v) \quad (4859)$$

$$\tau_{\gamma,\delta,w}^3 = \sum_{\epsilon \in A} Z_{\delta,\epsilon}^* \tau_{\gamma,\epsilon,w}^1 \tau_{\gamma,\epsilon,w}^2 \quad (3r_D r_T^3) \quad (4847)$$

$$\tau_{\gamma,\delta,w}^1 = \sum_{a \in V} {}^2D_{a,w}^3 Y_{a,\gamma}^3 Y_{a,\delta}^{3,*} \quad (3r_D r_T^2 N_v) \quad (4860)$$

$$\tau^2_{\gamma,\alpha} = \sum_{a \in V} W^4_{a,\alpha} Y^1_{a,\gamma} \quad (2r_T r_V N_v) \quad (4861)$$

$$\tau^1_{\gamma,\delta,w} = \sum_{a \in V} {}^2D^3_{a,w} Y^3_{a,\gamma} Y^{3,*}_{a,\delta} \quad (3r_D r_T^2 N_v) \quad (4874)$$

$$\tau^3_{\gamma,\alpha} = \sum_{a \in V} W^2_{a,\alpha} Y^3_{a,\gamma} \quad (2r_T r_V N_v) \quad (4862)$$

$$\tau^2_{\gamma,\alpha} = \sum_{a \in V} W^4_{a,\alpha} Y^1_{a,\gamma} \quad (2r_T r_V N_v) \quad (4875)$$

$$\tau^4_{\gamma,\alpha} = \sum_{i \in O} W^1_{i,\alpha} Y^4_{i,\gamma} \quad (2r_T r_V N_o) \quad (4863)$$

$$\tau^3_{\gamma,\alpha} = \sum_{i \in O} W^3_{i,\alpha} Y^2_{i,\gamma} \quad (2r_T r_V N_o) \quad (4876)$$

$$\tau^5_{\gamma,\alpha} = \sum_{\beta \in B} X_{\beta,\alpha} \tau^3_{\gamma,\beta} \tau^4_{\gamma,\beta} \quad (3r_T r_V^2) \quad (4864)$$

$$\tau^4_{\gamma,\alpha} = \sum_{\beta \in B} X_{\alpha,\beta} \tau^2_{\gamma,\beta} \tau^3_{\gamma,\beta} \quad (3r_T r_V^2) \quad (4877)$$

$$\tau^6_{\gamma,\alpha} = \sum_{\delta \in A} Z_{\gamma,\delta} \tau^5_{\delta,\alpha} \quad (2r_T^2 r_V) \quad (4865)$$

$$\tau^5_{\gamma,\alpha} = \sum_{\delta \in A} Z_{\delta,\gamma} \tau^4_{\delta,\alpha} \quad (2r_T^2 r_V) \quad (4878)$$

$$\tau^7_{\gamma,\delta,i} = \sum_{\alpha \in B} W^3_{i,\alpha} \tau^2_{\gamma,\alpha} \tau^6_{\delta,\alpha} \quad (3r_T^2 r_V N_o) \quad (4866)$$

$$\tau^6_{\gamma,\alpha} = \sum_{a \in V} W^2_{a,\alpha} Y^3_{a,\gamma} \quad (2r_T r_V N_v) \quad (4879)$$

$$\tau^8_{\gamma,\delta,\epsilon} = \sum_{i \in O} Z_{\gamma,\epsilon} Y^4_{i,\epsilon} \tau^7_{\gamma,\delta,i} \quad (3r_T^3 N_o) \quad (4867)$$

$$\tau^7_{\gamma,i} = \sum_{\alpha \in B} W^1_{i,\alpha} \tau^5_{\gamma,\alpha} \tau^6_{\gamma,\alpha} \quad (3r_T r_V N_o) \quad (4880)$$

$$\tau^9_{\gamma,\delta,i} = \sum_{\epsilon \in A} Y^2_{i,\epsilon} \tau^8_{\epsilon,\gamma,\delta} \quad (2r_T^3 N_o) \quad (4868)$$

$$\tau^8_{i,j} = \sum_{\gamma \in A} Y^4_{j,\gamma} \tau^7_{\gamma,i} \quad (2r_T N_o^2) \quad (4881)$$

$$\tau^{10}_{\gamma,\delta,w} = \sum_{\epsilon \in A} \sum_{i \in O} {}^2D^4_{i,w} Y^{4,*}_{i,\delta} \tau^1_{\epsilon,\delta,w} \tau^9_{\gamma,\epsilon,i} \quad (4r_D r_T^3 N_o) \quad (4869)$$

$$\tau^9_{\gamma,i} = \sum_{j \in O} Y^4_{j,\gamma} \tau^8_{j,i} \quad (2r_T N_o^2) \quad (4882)$$

$$\tau^{11}_{\gamma,\delta,w} = \sum_{\epsilon \in A} Z^*_{\delta,\epsilon} \tau^{10}_{\gamma,\epsilon,w} \quad (2r_D r_T^3) \quad (4870)$$

$$\tau^{10}_{\gamma,\delta,w} = \sum_{i \in O} {}^2D^4_{i,w} Y^{4,*}_{i,\delta} \tau^9_{\gamma,i} \quad (3r_D r_T^2 N_o) \quad (4883)$$

$$\tau^{11}_{\gamma,\delta,w} = \sum_{\epsilon \in A} Z^*_{\delta,\epsilon} \tau^1_{\gamma,\epsilon,w} \tau^{10}_{\gamma,\epsilon,w} \quad (3r_D r_T^3) \quad (4884)$$

$${}^2R^2_{i,\gamma} \leftarrow - \sum_{\delta \in A} \sum_{w \in D} \frac{1}{2} {}^2D^2_{i,w} Y^2_{i,\delta} \tau^0_{\delta,\gamma,w} \tau^{11}_{\delta,\gamma,w} \quad (4r_D r_T^2 N_o) \quad (4871)$$

$$\tau^{12}_{\gamma,\delta,w} = \sum_{\epsilon \in A} Z_{\gamma,\epsilon} \tau^{11}_{\epsilon,\delta,w} \quad (2r_D r_T^3) \quad (4885)$$

Raw expression

$${}^2R^2_{i,\epsilon} \leftarrow - \sum_{\gamma \in A} \sum_{j \in O} \sum_{k \in O} \sum_{l \in O} \sum_{a \in V} \sum_{b \in V} \sum_{c \in V} \sum_{d \in V} \frac{1}{2} \quad (4872)$$

$$Y^{1,*}_{a,\epsilon} Z^*_{\epsilon,\gamma} Y^{3,*}_{b,\gamma} Y^{4,*}_{j,\gamma} {}^2D^{a,i,b,j} {}^2T_{a,i,c,k} {}^2T_{d,l,b,j} V_{k,d,l,c}$$

$${}^2R^2_{i,\gamma} \leftarrow - \sum_{\delta \in A} \sum_{w \in D} \frac{1}{2} {}^2D^2_{i,w} Y^2_{i,\delta} \tau^0_{\delta,\gamma,w} \tau^{12}_{\delta,\gamma,w} \quad (4r_D r_T^2 N_o) \quad (4886)$$

Raw expression

Factorized expression

$$\tau^0_{\gamma,\delta,w} = \sum_{a \in V} {}^2D^1_{a,w} Y^1_{a,\gamma} Y^{1,*}_{a,\delta} \quad (3r_D r_T^2 N_v) \quad (4873)$$

$${}^2R^2_{i,\epsilon} \leftarrow - \sum_{\gamma \in A} \sum_{j \in O} \sum_{k \in O} \sum_{l \in O} \sum_{a \in V} \sum_{b \in V} \sum_{c \in V} \sum_{d \in V} \frac{1}{2} \quad (4887)$$

$$Y^{1,*}_{a,\epsilon} Z^*_{\epsilon,\gamma} Y^{3,*}_{b,\gamma} Y^{4,*}_{j,\gamma} {}^2D^{a,i,b,j} {}^2T_{a,k,c,i} {}^2T_{b,j,d,l} V_{k,c,l,d}$$



Factorized expression

$$\tau_{\gamma,\delta,w}^0 = \sum_{a \in V} {}^2D_{a,w}^1 Y_{a,\gamma}^1 Y_{a,\delta}^{1,*} \quad (3r_D r_T^2 N_v) \quad (4888)$$

$$\tau_{\gamma,\delta,w}^1 = \sum_{a \in V} {}^2D_{a,w}^3 Y_{a,\gamma}^3 Y_{a,\delta}^{3,*} \quad (3r_D r_T^2 N_v) \quad (4889)$$

$$\tau_{\gamma,\delta,w}^2 = \sum_{i \in O} {}^2D_{i,w}^4 Y_{i,\gamma}^4 Y_{i,\delta}^{4,*} \quad (3r_D r_T^2 N_o) \quad (4890)$$

$$\tau_{\gamma,\delta,w}^3 = \sum_{\epsilon \in A} Z_{\delta,\epsilon}^* \tau_{\gamma,\epsilon,w}^1 \tau_{\gamma,\epsilon,w}^2 \quad (3r_D r_T^3) \quad (4891)$$

$$\tau_{\gamma,\delta,w}^4 = \sum_{\epsilon \in A} Z_{\gamma,\epsilon} \tau_{\epsilon,\delta,w}^3 \quad (2r_D r_T^3) \quad (4892)$$

$$\tau_{\gamma,\alpha}^5 = \sum_{a \in V} W_{a,\alpha}^4 Y_{a,\gamma}^1 \quad (2r_T r_V N_v) \quad (4893)$$

$$\tau_{\gamma,\alpha}^6 = \sum_{i \in O} W_{i,\alpha}^3 Y_{i,\gamma}^2 \quad (2r_T r_V N_o) \quad (4894)$$

$$\tau_{\gamma,\alpha}^7 = \sum_{\beta \in B} X_{\alpha,\beta} \tau_{\gamma,\beta}^5 \tau_{\gamma,\beta}^6 \quad (3r_T r_V^2) \quad (4895)$$

$$\tau_{\gamma,\alpha}^8 = \sum_{\delta \in A} Z_{\delta,\gamma} \tau_{\delta,\alpha}^7 \quad (2r_T^2 r_V) \quad (4896)$$

$$\tau_{\gamma,\alpha}^9 = \sum_{a \in V} W_{a,\alpha}^2 Y_{a,\gamma}^3 \quad (2r_T r_V N_v) \quad (4897)$$

$$\tau_{\gamma,i}^{10} = \sum_{\alpha \in B} W_{i,\alpha}^1 \tau_{\gamma,\alpha}^8 \tau_{\gamma,\alpha}^9 \quad (3r_T r_V N_o) \quad (4898)$$

$$\tau_{i,j}^{11} = \sum_{\gamma \in A} Y_{j,\gamma}^4 \tau_{\gamma,i}^{10} \quad (2r_T N_o^2) \quad (4899)$$

$$\tau_{\gamma,i}^{12} = \sum_{j \in O} Y_{j,\gamma}^2 \tau_{j,i}^{11} \quad (2r_T N_o^2) \quad (4900)$$

$${}^2R_{i,\gamma}^2 \leftarrow - \sum_{\delta \in A} \sum_{w \in D} \frac{1}{2} {}^2D_{i,w}^2 \tau_{\delta,i}^{12} \tau_{\delta,\gamma,w}^0 \tau_{\delta,\gamma,w}^4 \quad (4r_D r_T^2 N_o) \quad (4901)$$

Raw expression

$${}^2R_{i,\epsilon}^2 \leftarrow - \sum_{\gamma \in A} \sum_{j \in O} \sum_{k \in O} \sum_{l \in O} \sum_{a \in V} \sum_{b \in V} \sum_{c \in V} \sum_{d \in V} \frac{1}{2} \quad (4902)$$

$$Y_{a,\epsilon}^{1,*} Z_{\epsilon,\gamma}^* Y_{b,\gamma}^{3,*} Y_{j,\gamma}^{4,*} {}^2D_{a,i,b,j} {}^2T_{a,k,c,i} {}^2T_{d,l,b,j} V_{k,c,l,d}$$

Factorized expression

$$\tau_{\gamma,\delta,w}^0 = \sum_{a \in V} {}^2D_{a,w}^1 Y_{a,\gamma}^1 Y_{a,\delta}^{1,*} \quad (3r_D r_T^2 N_v) \quad (4903)$$

$$\tau_{\gamma,\delta,w}^1 = \sum_{a \in V} {}^2D_{a,w}^3 Y_{a,\gamma}^3 Y_{a,\delta}^{3,*} \quad (3r_D r_T^2 N_v) \quad (4904)$$

$$\tau_{\gamma,\delta,w}^2 = \sum_{i \in O} {}^2D_{i,w}^4 Y_{i,\gamma}^4 Y_{i,\delta}^{4,*} \quad (3r_D r_T^2 N_o) \quad (4905)$$

$$\tau_{\gamma,\delta,w}^3 = \sum_{\epsilon \in A} Z_{\delta,\epsilon}^* \tau_{\gamma,\epsilon,w}^1 \tau_{\gamma,\epsilon,w}^2 \quad (3r_D r_T^3) \quad (4906)$$

$$\tau_{\gamma,\alpha}^4 = \sum_{a \in V} W_{a,\alpha}^2 Y_{a,\gamma}^3 \quad (2r_T r_V N_v) \quad (4907)$$

$$\tau_{\gamma,\alpha}^5 = \sum_{a \in V} W_{a,\alpha}^4 Y_{a,\gamma}^1 \quad (2r_T r_V N_v) \quad (4908)$$

$$\tau_{\gamma,\alpha}^6 = \sum_{i \in O} W_{i,\alpha}^3 Y_{i,\gamma}^2 \quad (2r_T r_V N_o) \quad (4909)$$

$$\tau_{\gamma,\alpha}^7 = \sum_{\beta \in B} X_{\alpha,\beta} \tau_{\gamma,\beta}^5 \tau_{\gamma,\beta}^6 \quad (3r_T r_V^2) \quad (4910)$$

$$\tau_{\gamma,\alpha}^8 = \sum_{\delta \in A} Z_{\delta,\gamma} \tau_{\delta,\alpha}^7 \quad (2r_T^2 r_V) \quad (4911)$$

$$\tau_{\gamma,\delta,i}^9 = \sum_{\alpha \in B} W_{i,\alpha}^1 \tau_{\delta,\alpha}^4 \tau_{\gamma,\alpha}^8 \quad (3r_T^2 r_V N_o) \quad (4912)$$

$$\tau_{\gamma,\delta,\epsilon}^{10} = \sum_{i \in O} Y_{i,\gamma}^2 \tau_{\delta,\epsilon,i}^9 \quad (2r_T^3 N_o) \quad (4913)$$

$$\tau_{\gamma,\delta,i}^{11} = \sum_{\epsilon \in A} Z_{\gamma,\epsilon} Y_{i,\epsilon}^4 \tau_{\gamma,\delta,\epsilon}^{10} \quad (3r_T^3 N_o) \quad (4914)$$

$$\tau_{\gamma,\delta,w,i}^{12} = \sum_{\epsilon \in A} \tau_{\gamma,\epsilon,i}^{11} \tau_{\epsilon,\delta,w}^3 \quad (2r_D r_T^3 N_o) \quad (4915)$$

$$\tau^{13}_{\gamma,w,i} = \sum_{\delta \in A} \tau^0_{\delta,\gamma,w} \tau^{12}_{\delta,\gamma,w,i} \quad (2r_D r_T^2 N_o) \quad (4916)$$

$$\tau^{10}_{\gamma,\delta,\epsilon} = \sum_{i \in O} Y^2_{i,\gamma} Z_{\gamma,\epsilon} \tau^9_{\delta,\epsilon,i} \quad (3r_T^3 N_o) \quad (4929)$$

$${}^2R^2_{i,\gamma} \leftarrow - \sum_{w \in D} \frac{1}{2} {}^2D^2_{i,w} \tau^{13}_{\gamma,w,i} \quad (2r_D r_T N_o) \quad (4917)$$

$$\tau^{11}_{\gamma,\delta,i} = \sum_{\epsilon \in A} Y^4_{i,\epsilon} \tau^{10}_{\gamma,\delta,\epsilon} \quad (2r_T^3 N_o) \quad (4930)$$

Raw expression

$${}^2R^2_{i,\epsilon} \leftarrow - \sum_{\gamma \in A} \sum_{j \in O} \sum_{k \in O} \sum_{l \in O} \sum_{a \in V} \sum_{b \in V} \sum_{c \in V} \sum_{d \in V} \frac{1}{2} \quad (4918)$$

$$Y^{1,*}_{a,\epsilon} \quad Z^{*,\gamma}_{\epsilon,\gamma} \quad Y^{3,*}_{b,\gamma} \quad Y^{4,*}_{j,\gamma} \quad {}^2D^{a,i,b,j}_{a,k,d,l} \quad {}^2T_{a,k,d,l} \quad {}^2T_{b,j,c,i} \quad V_{k,c,l,d}$$

$$\tau^{12}_{\gamma,\delta,w,i} = \sum_{\epsilon \in A} \tau^{11}_{\gamma,\epsilon,i} \tau^3_{\epsilon,\delta,w} \quad (2r_D r_T^3 N_o) \quad (4931)$$

$$\tau^{13}_{\gamma,w,i} = \sum_{\delta \in A} \tau^0_{\delta,\gamma,w} \tau^{12}_{\delta,\gamma,w,i} \quad (2r_D r_T^2 N_o) \quad (4932)$$

Factorized expression

$$\tau^0_{\gamma,\delta,w} = \sum_{a \in V} {}^2D^1_{a,w} Y^1_{a,\gamma} Y^{1,*}_{a,\delta} \quad (3r_D r_T^2 N_v) \quad (4919)$$

$${}^2R^2_{i,\gamma} \leftarrow - \sum_{w \in D} \frac{1}{2} {}^2D^2_{i,w} \tau^{13}_{\gamma,w,i} \quad (2r_D r_T N_o) \quad (4933)$$

Raw expression

$$\tau^1_{\gamma,\delta,w} = \sum_{a \in V} {}^2D^3_{a,w} Y^1_{a,\gamma} Y^{3,*}_{a,\delta} \quad (3r_D r_T^2 N_v) \quad (4920)$$

$${}^2R^2_{i,\epsilon} \leftarrow - \sum_{\gamma \in A} \sum_{j \in O} \sum_{k \in O} \sum_{l \in O} \sum_{a \in V} \sum_{b \in V} \sum_{c \in V} \sum_{d \in V} \frac{1}{2} \quad (4934)$$

$$Y^{1,*}_{a,\epsilon} \quad Z^{*,\gamma}_{\epsilon,\gamma} \quad Y^{3,*}_{b,\gamma} \quad Y^{4,*}_{j,\gamma} \quad {}^2D^{a,i,b,j}_{a,k,d,l} \quad {}^2T_{a,k,d,l} \quad {}^2T_{c,i,b,j} \quad V_{k,c,l,d}$$

$$\tau^2_{\gamma,\delta,w} = \sum_{i \in O} {}^2D^4_{i,w} Y^2_{i,\gamma} Y^{4,*}_{i,\delta} \quad (3r_D r_T^2 N_o) \quad (4921)$$

Factorized expression

$$\tau^3_{\gamma,\delta,w} = \sum_{\epsilon \in A} Z^*_{\delta,\epsilon} \tau^1_{\gamma,\epsilon,w} \tau^2_{\gamma,\epsilon,w} \quad (3r_D r_T^3) \quad (4922)$$

$$\tau^0_{\gamma,\delta,w} = \sum_{a \in V} {}^2D^3_{a,w} Y^1_{a,\gamma} Y^{3,*}_{a,\delta} \quad (3r_D r_T^2 N_v) \quad (4935)$$

$$\tau^4_{\gamma,\alpha} = \sum_{a \in V} W^4_{a,\alpha} Y^3_{a,\gamma} \quad (2r_T r_V N_v) \quad (4923)$$

$$\tau^1_{\gamma,\delta,w} = \sum_{i \in O} {}^2D^4_{i,w} Y^2_{i,\gamma} Y^{4,*}_{i,\delta} \quad (3r_D r_T^2 N_o) \quad (4936)$$

$$\tau^5_{\gamma,\alpha} = \sum_{i \in O} W^3_{i,\alpha} Y^4_{i,\gamma} \quad (2r_T r_V N_o) \quad (4924)$$

$$\tau^2_{\gamma,\delta,w} = \sum_{\epsilon \in A} Z^*_{\delta,\epsilon} \tau^0_{\gamma,\epsilon,w} \tau^1_{\gamma,\epsilon,w} \quad (3r_D r_T^3) \quad (4937)$$

$$\tau^6_{\gamma,\alpha} = \sum_{\beta \in B} X_{\alpha,\beta} \tau^4_{\gamma,\beta} \tau^5_{\gamma,\beta} \quad (3r_T r_V^2) \quad (4925)$$

$$\tau^3_{\gamma,\delta,w} = \sum_{\epsilon \in A} Z_{\epsilon,\gamma} \tau^2_{\epsilon,\delta,w} \quad (2r_D r_T^3) \quad (4938)$$

$$\tau^7_{\gamma,\alpha} = \sum_{\delta \in A} Z_{\gamma,\delta} \tau^6_{\delta,\alpha} \quad (2r_T^2 r_V) \quad (4926)$$

$$\tau^4_{\gamma,\alpha} = \sum_{i \in O} W^1_{i,\alpha} Y^2_{i,\gamma} \quad (2r_T r_V N_o) \quad (4939)$$

$$\tau^8_{\gamma,\alpha} = \sum_{a \in V} W^2_{a,\alpha} Y^3_{a,\gamma} \quad (2r_T r_V N_v) \quad (4927)$$

$$\tau^5_{\gamma,\alpha} = \sum_{a \in V} W^4_{a,\alpha} Y^3_{a,\gamma} \quad (2r_T r_V N_v) \quad (4940)$$

$$\tau^9_{\gamma,\delta,i} = \sum_{\alpha \in B} W^1_{i,\alpha} \tau^7_{\gamma,\alpha} \tau^8_{\delta,\alpha} \quad (3r_T^2 r_V N_o) \quad (4928)$$

$$\tau^6_{\gamma,\alpha} = \sum_{i \in O} W^3_{i,\alpha} Y^4_{i,\gamma} \quad (2r_T r_V N_o) \quad (4941)$$

$$\tau^7_{\gamma,\alpha} = \sum_{\beta \in B} X_{\alpha,\beta} \tau^5_{\gamma,\beta} \tau^6_{\gamma,\beta} \quad (3r_T r_V^2) \quad (4942)$$

$$\tau^5_{\gamma,\alpha} = \sum_{a \in V} W^2_{a,\alpha} Y^1_{a,\gamma} \quad (2r_T r_V N_v) \quad (4955)$$

$$\tau^8_{\gamma,\alpha} = \sum_{\delta \in A} Z_{\gamma,\delta} \tau^7_{\delta,\alpha} \quad (2r_T^2 r_V) \quad (4943)$$

$$\tau^6_{\gamma,\alpha} = \sum_{a \in V} W^4_{a,\alpha} Y^3_{a,\gamma} \quad (2r_T r_V N_v) \quad (4956)$$

$$\tau^9_{\gamma,a} = \sum_{\alpha \in B} W^2_{a,\alpha} \tau^4_{\gamma,\alpha} \tau^8_{\gamma,\alpha} \quad (3r_T r_V N_v) \quad (4944)$$

$$\tau^7_{\gamma,\alpha} = \sum_{i \in O} W^3_{i,\alpha} Y^4_{i,\gamma} \quad (2r_T r_V N_o) \quad (4957)$$

$$\tau^{10}_{a,b} = \sum_{\gamma \in A} Y^1_{b,\gamma} \tau^9_{\gamma,a} \quad (2r_T N_v^2) \quad (4945)$$

$$\tau^8_{\gamma,\alpha} = \sum_{\beta \in B} X_{\alpha,\beta} \tau^6_{\gamma,\beta} \tau^7_{\gamma,\beta} \quad (3r_T r_V^2) \quad (4958)$$

$$\tau^{11}_{\gamma,a} = \sum_{b \in V} Y^3_{b,\gamma} \tau^{10}_{b,a} \quad (2r_T N_v^2) \quad (4946)$$

$$\tau^9_{\gamma,\alpha} = \sum_{\delta \in A} Z_{\gamma,\delta} \tau^8_{\delta,\alpha} \quad (2r_T^2 r_V) \quad (4959)$$

$$\tau^{12}_{\gamma,\delta,w} = \sum_{a \in V} {}^2D^1_{a,w} Y^{1,*}_{a,\delta} \tau^{11}_{\gamma,a} \quad (3r_D r_T^2 N_v) \quad (4947)$$

$$\tau^{10}_{\gamma,i} = \sum_{\alpha \in B} W^1_{i,\alpha} \tau^5_{\gamma,\alpha} \tau^9_{\gamma,\alpha} \quad (3r_T r_V N_o) \quad (4960)$$

$${}^2R^2_{i,\gamma} \leftarrow - \sum_{\delta \in A} \sum_{w \in D} \frac{1}{2} {}^2D^2_{i,w} Y^4_{i,\delta} \tau^{12}_{\delta,\gamma,w} \tau^3_{\delta,\gamma,w} \quad (4r_D r_T^2 N_o) \quad (4948)$$

$$\tau^{11}_{i,j} = \sum_{\gamma \in A} Y^2_{j,\gamma} \tau^{10}_{\gamma,i} \quad (2r_T N_o^2) \quad (4961)$$

Raw expression

$$\tau^{12}_{\gamma,i} = \sum_{j \in O} Y^2_{j,\gamma} \tau^{11}_{j,i} \quad (2r_T N_o^2) \quad (4962)$$

$${}^2R^2_{i,\epsilon} \leftarrow - \sum_{\gamma \in A} \sum_{j \in O} \sum_{k \in O} \sum_{l \in O} \sum_{a \in V} \sum_{b \in V} \sum_{c \in V} \sum_{d \in V} \frac{1}{2} \quad (4949)$$

$$\begin{array}{l} Y^{1,*}_{a,\epsilon} \quad Z^*_{\epsilon,\gamma} \quad Y^{3,*}_{b,\gamma} \quad Y^{4,*}_{j,\gamma} \\ {}^2D^{a,i,b,j} \quad {}^2T_{a,l,b,j} \quad {}^2T_{c,i,d,k} \quad V_{l,c,k,d} \end{array}$$

$${}^2R^2_{i,\gamma} \leftarrow - \sum_{\delta \in A} \sum_{w \in D} \frac{1}{2} {}^2D^2_{i,w} \tau^{12}_{\delta,i} \tau^0_{\delta,\gamma,w} \tau^4_{\delta,\gamma,w} \quad (4r_D r_T^2 N_o) \quad (4963)$$

Factorized expression

Raw expression

$$\tau^0_{\gamma,\delta,w} = \sum_{a \in V} {}^2D^1_{a,w} Y^1_{a,\gamma} Y^{1,*}_{a,\delta} \quad (3r_D r_T^2 N_v) \quad (4950)$$

$${}^2R^2_{i,\epsilon} \leftarrow - \sum_{\gamma \in A} \sum_{j \in O} \sum_{k \in O} \sum_{l \in O} \sum_{a \in V} \sum_{b \in V} \sum_{c \in V} \sum_{d \in V} \frac{1}{2} \quad (4964)$$

$$\begin{array}{l} Y^{1,*}_{a,\epsilon} \quad Z^*_{\epsilon,\gamma} \quad Y^{3,*}_{b,\gamma} \quad Y^{4,*}_{j,\gamma} \\ {}^2D^{a,i,b,j} \quad {}^2T_{a,l,b,j} \quad {}^2T_{c,k,d,i} \quad V_{l,d,k,c} \end{array}$$

$$\tau^1_{\gamma,\delta,w} = \sum_{a \in V} {}^2D^3_{a,w} Y^3_{a,\gamma} Y^{3,*}_{a,\delta} \quad (3r_D r_T^2 N_v) \quad (4951)$$

Factorized expression

$$\tau^2_{\gamma,\delta,w} = \sum_{i \in O} {}^2D^4_{i,w} Y^4_{i,\gamma} Y^{4,*}_{i,\delta} \quad (3r_D r_T^2 N_o) \quad (4952)$$

$$\tau^0_{\gamma,\alpha} = \sum_{i \in O} W^1_{i,\alpha} Y^2_{i,\gamma} \quad (2r_T r_V N_o) \quad (4965)$$

$$\tau^3_{\gamma,\delta,w} = \sum_{\epsilon \in A} Z^*_{\delta,\epsilon} \tau^1_{\gamma,\epsilon,w} \tau^2_{\gamma,\epsilon,w} \quad (3r_D r_T^3) \quad (4953)$$

$$\tau^1_{\gamma,\alpha} = \sum_{a \in V} W^4_{a,\alpha} Y^3_{a,\gamma} \quad (2r_T r_V N_v) \quad (4966)$$

$$\tau^4_{\gamma,\delta,w} = \sum_{\epsilon \in A} Z_{\gamma,\epsilon} \tau^3_{\epsilon,\delta,w} \quad (2r_D r_T^3) \quad (4954)$$

$$\tau^2_{\gamma,\alpha} = \sum_{i \in O} W^3_{i,\alpha} Y^4_{i,\gamma} \quad (2r_T r_V N_o) \quad (4967)$$

$$\tau^3_{\gamma,\alpha} = \sum_{\beta \in B} X_{\alpha,\beta} \tau^1_{\gamma,\beta} \tau^2_{\gamma,\beta} \quad (3r_T r_V^2) \quad (4968)$$

$$\tau^4_{\gamma,\alpha} = \sum_{\delta \in A} Z_{\gamma,\delta} \tau^3_{\delta,\alpha} \quad (2r_T^2 r_V) \quad (4969)$$

$$\tau^5_{\gamma,a} = \sum_{\alpha \in B} W^2_{a,\alpha} \tau^0_{\gamma,\alpha} \tau^4_{\gamma,\alpha} \quad (3r_T r_V N_v) \quad (4970)$$

$$\tau^6_{a,b} = \sum_{\gamma \in A} Y^1_{b,\gamma} \tau^5_{\gamma,a} \quad (2r_T N_v^2) \quad (4971)$$

$$\tau^7_{\gamma,a} = \sum_{b \in V} Y^1_{b,\gamma} \tau^6_{b,a} \quad (2r_T N_v^2) \quad (4972)$$

$$\tau^8_{\gamma,\delta,w} = \sum_{a \in V} {}^2D^1_{a,w} Y^{1,*}_{a,\delta} \tau^7_{\gamma,a} \quad (3r_D r_T^2 N_v) \quad (4973)$$

$$\tau^9_{\gamma,\delta,w} = \sum_{a \in V} {}^2D^3_{a,w} Y^3_{a,\gamma} Y^{3,*}_{a,\delta} \quad (3r_D r_T^2 N_v) \quad (4974)$$

$$\tau^{10}_{\gamma,\delta,w} = \sum_{i \in O} {}^2D^4_{i,w} Y^4_{i,\gamma} Y^{4,*}_{i,\delta} \quad (3r_D r_T^2 N_o) \quad (4975)$$

$$\tau^{11}_{\gamma,\delta,w} = \sum_{\epsilon \in A} Z^*_{\delta,\epsilon} \tau^{10}_{\gamma,\epsilon,w} \tau^9_{\gamma,\epsilon,w} \quad (3r_D r_T^3) \quad (4976)$$

$$\tau^{12}_{\gamma,\delta,w} = \sum_{\epsilon \in A} Z_{\gamma,\epsilon} \tau^{11}_{\epsilon,\delta,w} \quad (2r_D r_T^3) \quad (4977)$$

$${}^2R^2_{i,\gamma} \leftarrow - \sum_{\delta \in A} \sum_{w \in D} \frac{1}{2} {}^2D^2_{i,w} Y^2_{i,\delta} \tau^{12}_{\delta,\gamma,w} \tau^8_{\delta,\gamma,w} \quad (4r_D r_T^2 N_o) \quad (4978)$$

Raw expression

$${}^2R^2_{i,\epsilon} \leftarrow - \sum_{\gamma \in A} \sum_{j \in O} \sum_{k \in O} \sum_{l \in O} \sum_{a \in V} \sum_{b \in V} \sum_{c \in V} \sum_{d \in V} \frac{1}{2} Y^{1,*}_{a,\epsilon} Z^*_{\epsilon,\gamma} Y^{3,*}_{b,\gamma} Y^{4,*}_{j,\gamma} {}^2D^{a,i,b,j} {}^2T_{b,j,a,l} {}^2T_{c,i,d,k} V_{l,c,k,d} \quad (4979)$$

Factorized expression

$$\tau^0_{\gamma,\delta,w} = \sum_{a \in V} {}^2D^3_{a,w} Y^1_{a,\gamma} Y^{3,*}_{a,\delta} \quad (3r_D r_T^2 N_v) \quad (4980)$$

$$\tau^1_{\gamma,\delta,w} = \sum_{i \in O} {}^2D^4_{i,w} Y^2_{i,\gamma} Y^{4,*}_{i,\delta} \quad (3r_D r_T^2 N_o) \quad (4981)$$

$$\tau^2_{\gamma,\delta,w} = \sum_{\epsilon \in A} Z^*_{\delta,\epsilon} \tau^0_{\gamma,\epsilon,w} \tau^1_{\gamma,\epsilon,w} \quad (3r_D r_T^3) \quad (4982)$$

$$\tau^3_{\gamma,\delta,w} = \sum_{\epsilon \in A} Z_{\epsilon,\gamma} \tau^2_{\epsilon,\delta,w} \quad (2r_D r_T^3) \quad (4983)$$

$$\tau^4_{\gamma,\alpha} = \sum_{a \in V} W^2_{a,\alpha} Y^1_{a,\gamma} \quad (2r_T r_V N_v) \quad (4984)$$

$$\tau^5_{\gamma,\alpha} = \sum_{i \in O} W^1_{i,\alpha} Y^2_{i,\gamma} \quad (2r_T r_V N_o) \quad (4985)$$

$$\tau^6_{\gamma,\alpha} = \sum_{\beta \in B} X_{\beta,\alpha} \tau^4_{\gamma,\beta} \tau^5_{\gamma,\beta} \quad (3r_T r_V^2) \quad (4986)$$

$$\tau^7_{\gamma,\alpha} = \sum_{\delta \in A} Z_{\delta,\gamma} \tau^6_{\delta,\alpha} \quad (2r_T^2 r_V) \quad (4987)$$

$$\tau^8_{\gamma,\alpha} = \sum_{i \in O} W^3_{i,\alpha} Y^4_{i,\gamma} \quad (2r_T r_V N_o) \quad (4988)$$

$$\tau^9_{\gamma,a} = \sum_{\alpha \in B} W^4_{a,\alpha} \tau^7_{\gamma,\alpha} \tau^8_{\gamma,\alpha} \quad (3r_T r_V N_v) \quad (4989)$$

$$\tau^{10}_{\gamma,\delta} = \sum_{a \in V} Y^3_{a,\delta} \tau^9_{\gamma,a} \quad (2r_T^2 N_v) \quad (4990)$$

$$\tau^{11}_{\gamma,a} = \sum_{\delta \in A} Y^3_{a,\delta} \tau^{10}_{\delta,\gamma} \quad (2r_T^2 N_v) \quad (4991)$$

$$\tau^{12}_{\gamma,\delta,w} = \sum_{a \in V} {}^2D^1_{a,w} Y^{1,*}_{a,\delta} \tau^{11}_{\gamma,a} \quad (3r_D r_T^2 N_v) \quad (4992)$$

$${}^2R^2_{i,\gamma} \leftarrow - \sum_{\delta \in A} \sum_{w \in D} \frac{1}{2} {}^2D^2_{i,w} Y^4_{i,\delta} \tau^{12}_{\delta,\gamma,w} \tau^3_{\delta,\gamma,w} \quad (4r_D r_T^2 N_o) \quad (4993)$$

Raw expression

$${}^2R^2_{i,\epsilon} \leftarrow - \sum_{\gamma \in A} \sum_{j \in O} \sum_{k \in O} \sum_{l \in O} \sum_{a \in V} \sum_{b \in V} \sum_{c \in V} \sum_{d \in V} \frac{1}{2} Y^{1,*}_{a,\epsilon} Z^*_{\epsilon,\gamma} Y^{3,*}_{b,\gamma} Y^{4,*}_{j,\gamma} {}^2D^{a,i,b,j} {}^2T_{b,j,a,l} {}^2T_{c,k,d,i} V_{l,d,k,c} \quad (4994)$$

Factorized expression

$$\tau_{\gamma,\delta,w}^0 = \sum_{a \in V} {}^2D_{a,w}^1 Y_{a,\gamma}^3 Y_{a,\delta}^{1,*} \quad (3r_D r_T^2 N_v) \quad (4995)$$

$$\tau_{\gamma,\delta,w}^1 = \sum_{i \in O} {}^2D_{i,w}^4 Y_{i,\gamma}^2 Y_{i,\delta}^{4,*} \quad (3r_D r_T^2 N_o) \quad (4996)$$

$$\tau_{\gamma,\alpha}^2 = \sum_{i \in O} W_{i,\alpha}^1 Y_{i,\gamma}^2 \quad (2r_T r_V N_o) \quad (4997)$$

$$\tau_{\gamma,\alpha}^3 = \sum_{a \in V} W_{a,\alpha}^4 Y_{a,\gamma}^3 \quad (2r_T r_V N_v) \quad (4998)$$

$$\tau_{\gamma,\alpha}^4 = \sum_{i \in O} W_{i,\alpha}^3 Y_{i,\gamma}^4 \quad (2r_T r_V N_o) \quad (4999)$$

$$\tau_{\gamma,\alpha}^5 = \sum_{\beta \in B} X_{\alpha,\beta} \tau_{\gamma,\beta}^3 \tau_{\gamma,\beta}^4 \quad (3r_T r_V^2) \quad (5000)$$

$$\tau_{\gamma,\alpha}^6 = \sum_{\delta \in A} Z_{\gamma,\delta} \tau_{\delta,\alpha}^5 \quad (2r_T^2 r_V) \quad (5001)$$

$$\tau_{\gamma,a}^7 = \sum_{\alpha \in B} W_{a,\alpha}^2 \tau_{\gamma,\alpha}^2 \tau_{\gamma,\alpha}^6 \quad (3r_T r_V N_v) \quad (5002)$$

$$\tau_{a,b}^8 = \sum_{\gamma \in A} Y_{b,\gamma}^1 \tau_{\gamma,a}^7 \quad (2r_T N_v^2) \quad (5003)$$

$$\tau_{\gamma,a}^9 = \sum_{b \in V} Y_{b,\gamma}^1 \tau_{b,a}^8 \quad (2r_T N_v^2) \quad (5004)$$

$$\tau_{\gamma,\delta,w}^{10} = \sum_{a \in V} {}^2D_{a,w}^3 Y_{a,\delta}^{3,*} \tau_{\gamma,a}^9 \quad (3r_D r_T^2 N_v) \quad (5005)$$

$$\tau_{\gamma,\delta,w}^{11} = \sum_{\epsilon \in A} Z_{\delta,\epsilon}^* \tau_{\gamma,\epsilon,w}^1 \tau_{\gamma,\epsilon,w}^{10} \quad (3r_D r_T^3) \quad (5006)$$

$$\tau_{\gamma,\delta,w}^{12} = \sum_{\epsilon \in A} Z_{\epsilon,\gamma} \tau_{\epsilon,\delta,w}^{11} \quad (2r_D r_T^3) \quad (5007)$$

$${}^2R_{i,\gamma}^2 \leftarrow - \sum_{\delta \in A} \sum_{w \in D} \frac{1}{2} {}^2D_{i,w}^2 Y_{i,\delta}^4 \tau_{\delta,\gamma,w}^0 \tau_{\delta,\gamma,w}^{12} \quad (4r_D r_T^2 N_o) \quad (5008)$$

Raw expression

$${}^2R_{i,\epsilon}^2 \leftarrow - \sum_{\gamma \in A} \sum_{j \in O} \sum_{k \in O} \sum_{l \in O} \sum_{a \in V} \sum_{b \in V} \sum_{c \in V} \sum_{d \in V} \frac{1}{2} \quad (5009)$$

$$Y_{a,\epsilon}^{1,*} Z_{\epsilon,\gamma}^* Y_{b,\gamma}^{3,*} Y_{j,\gamma}^{4,*} {}^2D_{a,i,b,j} {}^2T_{b,j,c,i} {}^2T_{d,k,a,l} V_{k,d,l,c}$$

Factorized expression

$$\tau_{\gamma,\delta,w}^0 = \sum_{a \in V} {}^2D_{a,w}^1 Y_{a,\gamma}^3 Y_{a,\delta}^{1,*} \quad (3r_D r_T^2 N_v) \quad (5010)$$

$$\tau_{\gamma,\alpha}^1 = \sum_{a \in V} W_{a,\alpha}^2 Y_{a,\gamma}^1 \quad (2r_T r_V N_v) \quad (5011)$$

$$\tau_{\gamma,\alpha}^2 = \sum_{a \in V} W_{a,\alpha}^4 Y_{a,\gamma}^3 \quad (2r_T r_V N_v) \quad (5012)$$

$$\tau_{\gamma,\alpha}^3 = \sum_{i \in O} W_{i,\alpha}^3 Y_{i,\gamma}^4 \quad (2r_T r_V N_o) \quad (5013)$$

$$\tau_{\gamma,\alpha}^4 = \sum_{\beta \in B} X_{\alpha,\beta} \tau_{\gamma,\beta}^2 \tau_{\gamma,\beta}^3 \quad (3r_T r_V^2) \quad (5014)$$

$$\tau_{\gamma,\alpha}^5 = \sum_{\delta \in A} Z_{\gamma,\delta} \tau_{\delta,\alpha}^4 \quad (2r_T^2 r_V) \quad (5015)$$

$$\tau_{\gamma,i}^6 = \sum_{\alpha \in B} W_{i,\alpha}^1 \tau_{\gamma,\alpha}^1 \tau_{\gamma,\alpha}^5 \quad (3r_T r_V N_o) \quad (5016)$$

$$\tau_{i,j}^7 = \sum_{\gamma \in A} Y_{j,\gamma}^2 \tau_{\gamma,i}^6 \quad (2r_T N_o^2) \quad (5017)$$

$$\tau_{\gamma,i}^8 = \sum_{j \in O} Y_{j,\gamma}^2 \tau_{j,i}^7 \quad (2r_T N_o^2) \quad (5018)$$

$$\tau_{\gamma,\delta,w}^9 = \sum_{i \in O} {}^2D_{i,w}^4 Y_{i,\delta}^{4,*} \tau_{\gamma,i}^8 \quad (3r_D r_T^2 N_o) \quad (5019)$$

$$\tau_{\gamma,\delta,w}^{10} = \sum_{a \in V} {}^2D_{a,w}^3 Y_{a,\gamma}^1 Y_{a,\delta}^{3,*} \quad (3r_D r_T^2 N_v) \quad (5020)$$

$$\tau_{\gamma,\delta,w}^{11} = \sum_{\epsilon \in A} Z_{\delta,\epsilon}^* \tau_{\gamma,\epsilon,w}^{10} \tau_{\gamma,\epsilon,w}^9 \quad (3r_D r_T^3) \quad (5021)$$

$$\tau^{12}_{\gamma,\delta,w} = \sum_{\epsilon \in A} Z_{\epsilon,\gamma} \tau^{11}_{\epsilon,\delta,w} \quad (2r_D r_T^3) \quad (5022)$$

$$\tau^{10}_{\gamma,\delta,w} = \sum_{\epsilon \in A} \sum_{i \in O} {}^2D^4_{i,w} Y^{4,*}_{i,\delta} \tau^{11}_{\epsilon,\delta,w} \tau^9_{\epsilon,\gamma,i} \quad (4r_D r_T^3 N_o) \quad (5035)$$

$${}^2R^2_{i,\gamma} \leftarrow - \sum_{\delta \in A} \sum_{w \in D} \frac{1}{2} {}^2D^2_{i,w} Y^4_{i,\delta} \tau^0_{\delta,\gamma,w} \tau^{12}_{\delta,\gamma,w} \quad (4r_D r_T^2 N_o) \quad (5023)$$

$$\tau^{11}_{\gamma,\delta,w} = \sum_{\epsilon \in A} Z^*_{\delta,\epsilon} \tau^{10}_{\gamma,\epsilon,w} \quad (2r_D r_T^3) \quad (5036)$$

Raw expression

$${}^2R^2_{i,\epsilon} \leftarrow - \sum_{\gamma \in A} \sum_{j \in O} \sum_{k \in O} \sum_{l \in O} \sum_{a \in V} \sum_{b \in V} \sum_{c \in V} \sum_{d \in V} \frac{1}{2} \quad (5024)$$

$$Y^{1,*}_{a,\epsilon} Z^*_{\epsilon,\gamma} Y^{3,*}_{b,\gamma} Y^{4,*}_{j,\gamma} {}^2D^{a,i,b,j} {}^2T_{b,j,d,l} {}^2T_{c,i,a,k} V_{k,c,l,d}$$

Factorized expression

$$\tau^0_{\gamma,\delta,w} = \sum_{a \in V} {}^2D^1_{a,w} Y^3_{a,\gamma} Y^{1,*}_{a,\delta} \quad (3r_D r_T^2 N_v) \quad (5025)$$

$$\tau^1_{\gamma,\delta,w} = \sum_{a \in V} {}^2D^3_{a,w} Y^1_{a,\gamma} Y^{3,*}_{a,\delta} \quad (3r_D r_T^2 N_v) \quad (5026)$$

$$\tau^2_{\gamma,\alpha} = \sum_{a \in V} W^4_{a,\alpha} Y^3_{a,\gamma} \quad (2r_T r_V N_v) \quad (5027)$$

$$\tau^3_{\gamma,\alpha} = \sum_{a \in V} W^2_{a,\alpha} Y^1_{a,\gamma} \quad (2r_T r_V N_v) \quad (5028)$$

$$\tau^4_{\gamma,\alpha} = \sum_{i \in O} W^1_{i,\alpha} Y^2_{i,\gamma} \quad (2r_T r_V N_o) \quad (5029)$$

$$\tau^5_{\gamma,\alpha} = \sum_{\beta \in B} X_{\beta,\alpha} \tau^3_{\gamma,\beta} \tau^4_{\gamma,\beta} \quad (3r_T r_V^2) \quad (5030)$$

$$\tau^6_{\gamma,\alpha} = \sum_{\delta \in A} Z_{\delta,\gamma} \tau^5_{\delta,\alpha} \quad (2r_T^2 r_V) \quad (5031)$$

$$\tau^7_{\gamma,\delta,i} = \sum_{\alpha \in B} W^3_{i,\alpha} \tau^2_{\delta,\alpha} \tau^6_{\gamma,\alpha} \quad (3r_T^2 r_V N_o) \quad (5032)$$

$$\tau^8_{\gamma,\delta,\epsilon} = \sum_{i \in O} Y^2_{i,\gamma} \tau^7_{\delta,\epsilon,i} \quad (2r_T^3 N_o) \quad (5033)$$

$$\tau^9_{\gamma,\delta,i} = \sum_{\epsilon \in A} Z_{\gamma,\epsilon} Y^4_{i,\epsilon} \tau^8_{\gamma,\delta,\epsilon} \quad (3r_T^3 N_o) \quad (5034)$$

$${}^2R^2_{i,\gamma} \leftarrow - \sum_{\delta \in A} \sum_{w \in D} \frac{1}{2} {}^2D^2_{i,w} Y^4_{i,\delta} \tau^0_{\delta,\gamma,w} \tau^{11}_{\delta,\gamma,w} \quad (4r_D r_T^2 N_o) \quad (5037)$$

Raw expression

$${}^2R^2_{i,\epsilon} \leftarrow - \sum_{\gamma \in A} \sum_{j \in O} \sum_{k \in O} \sum_{l \in O} \sum_{a \in V} \sum_{b \in V} \sum_{c \in V} \sum_{d \in V} \frac{1}{2} \quad (5038)$$

$$Y^{1,*}_{a,\epsilon} Z^*_{\epsilon,\gamma} Y^{3,*}_{b,\gamma} Y^{4,*}_{j,\gamma} {}^2D^{a,i,b,j} {}^2T_{b,j,d,l} {}^2T_{c,k,a,i} V_{k,d,l,c}$$

Factorized expression

$$\tau^0_{\gamma,\delta,w} = \sum_{a \in V} {}^2D^1_{a,w} Y^3_{a,\gamma} Y^{1,*}_{a,\delta} \quad (3r_D r_T^2 N_v) \quad (5039)$$

$$\tau^1_{\gamma,\delta,w} = \sum_{a \in V} {}^2D^3_{a,w} Y^1_{a,\gamma} Y^{3,*}_{a,\delta} \quad (3r_D r_T^2 N_v) \quad (5040)$$

$$\tau^2_{\gamma,\delta,w} = \sum_{i \in O} {}^2D^4_{i,w} Y^2_{i,\gamma} Y^{4,*}_{i,\delta} \quad (3r_D r_T^2 N_o) \quad (5041)$$

$$\tau^3_{\gamma,\delta,w} = \sum_{\epsilon \in A} Z^*_{\delta,\epsilon} \tau^1_{\gamma,\epsilon,w} \tau^2_{\gamma,\epsilon,w} \quad (3r_D r_T^3) \quad (5042)$$

$$\tau^4_{\gamma,\alpha} = \sum_{a \in V} W^2_{a,\alpha} Y^3_{a,\gamma} \quad (2r_T r_V N_v) \quad (5043)$$

$$\tau^5_{\gamma,\alpha,i} = \sum_{\beta \in B} W^1_{i,\beta} X_{\beta,\alpha} \tau^4_{\gamma,\beta} \quad (3r_T r_V^2 N_o) \quad (5044)$$

$$\tau^6_{\gamma,\alpha} = \sum_{i \in O} W^3_{i,\alpha} Y^4_{i,\gamma} \quad (2r_T r_V N_o) \quad (5045)$$

$$\tau^7_{\gamma,\alpha} = \sum_{a \in V} W^4_{a,\alpha} Y^1_{a,\gamma} \quad (2r_T r_V N_v) \quad (5046)$$

$$\tau^8_{\gamma,\delta,i} = \sum_{\alpha \in B} \tau^6_{\delta,\alpha} \tau^7_{\gamma,\alpha} \tau^5_{\delta,\alpha,i} \quad (3r_T^2 r_V N_o) \quad (5047)$$

$$\tau^9_{\gamma,\delta} = \sum_{i \in O} Y^2_{i,\gamma} \tau^8_{\gamma,\delta,i} \quad (2r_T^2 N_o) \quad (5048)$$

$$\tau^7_{\gamma,\alpha} = \sum_{\beta \in B} X_{\alpha,\beta} \tau^5_{\gamma,\beta} \tau^6_{\gamma,\beta} \quad (3r_T r_V^2) \quad (5061)$$

$$\tau^{10}_{\gamma,\delta} = \sum_{\epsilon \in A} Z_{\delta,\epsilon} \tau^9_{\gamma,\epsilon} \quad (2r_T^3) \quad (5049)$$

$$\tau^8_{\gamma,\alpha} = \sum_{\delta \in A} Z_{\delta,\gamma} \tau^7_{\delta,\alpha} \quad (2r_T^2 r_V) \quad (5062)$$

$$\tau^{11}_{\gamma,\delta} = \sum_{\epsilon \in A} Z_{\epsilon,\delta} \tau^{10}_{\epsilon,\gamma} \quad (2r_T^3) \quad (5050)$$

$$\tau^9_{\gamma,\alpha} = \sum_{a \in V} W^2_{a,\alpha} Y^3_{a,\gamma} \quad (2r_T r_V N_v) \quad (5063)$$

$$\tau^{12}_{\gamma,\delta,w} = \sum_{\epsilon \in A} \tau^{11}_{\epsilon,\gamma} \tau^3_{\epsilon,\delta,w} \quad (2r_D r_T^3) \quad (5051)$$

$$\tau^{10}_{\gamma,i} = \sum_{\alpha \in B} W^1_{i,\alpha} \tau^8_{\gamma,\alpha} \tau^9_{\gamma,\alpha} \quad (3r_T r_V N_o) \quad (5064)$$

$${}^2R^2_{i,\gamma} \leftarrow - \sum_{\delta \in A} \sum_{w \in D} \frac{1}{2} {}^2D^2_{i,w} Y^4_{i,\delta} \tau^0_{\delta,\gamma,w} \tau^{12}_{\delta,\gamma,w} \quad (4r_D r_T^2 N_o) \quad (5052)$$

$$\tau^{11}_{i,j} = \sum_{\gamma \in A} Y^4_{j,\gamma} \tau^{10}_{\gamma,i} \quad (2r_T N_o^2) \quad (5065)$$

Raw expression

$$\tau^{12}_{\gamma,i} = \sum_{j \in O} Y^4_{j,\gamma} \tau^{11}_{j,i} \quad (2r_T N_o^2) \quad (5066)$$

$${}^2R^2_{i,\epsilon} \leftarrow - \sum_{\gamma \in A} \sum_{j \in O} \sum_{k \in O} \sum_{l \in O} \sum_{a \in V} \sum_{b \in V} \sum_{c \in V} \sum_{d \in V} \frac{1}{2} \quad (5053)$$

$$Y^{1,*}_{a,\epsilon} Z^*_{\epsilon,\gamma} Y^{3,*}_{b,\gamma} Y^{4,*}_{j,\gamma} {}^2D^{a,i,b,j} {}^2T_{b,k,a,i} {}^2T_{c,j,d,l} V_{k,c,l,d}$$

$${}^2R^2_{i,\gamma} \leftarrow - \sum_{\delta \in A} \sum_{w \in D} \frac{1}{2} {}^2D^2_{i,w} \tau^{12}_{\delta,i} \tau^3_{\delta,\gamma,w} \tau^4_{\delta,\gamma,w} \quad (4r_D r_T^2 N_o) \quad (5067)$$

Factorized expression

Raw expression

$$\tau^0_{\gamma,\delta,w} = \sum_{a \in V} {}^2D^3_{a,w} Y^1_{a,\gamma} Y^{3,*}_{a,\delta} \quad (3r_D r_T^2 N_v) \quad (5054)$$

$${}^2R^2_{i,\epsilon} \leftarrow - \sum_{\gamma \in A} \sum_{j \in O} \sum_{k \in O} \sum_{l \in O} \sum_{a \in V} \sum_{b \in V} \sum_{c \in V} \sum_{d \in V} \frac{1}{2} \quad (5068)$$

$$Y^{1,*}_{a,\epsilon} Z^*_{\epsilon,\gamma} Y^{3,*}_{b,\gamma} Y^{4,*}_{j,\gamma} {}^2D^{a,i,b,j} {}^2T_{b,k,a,i} {}^2T_{c,l,d,j} V_{k,d,l,c}$$

$$\tau^1_{\gamma,\delta,w} = \sum_{i \in O} {}^2D^4_{i,w} Y^2_{i,\gamma} Y^{4,*}_{i,\delta} \quad (3r_D r_T^2 N_o) \quad (5055)$$

Factorized expression

$$\tau^2_{\gamma,\delta,w} = \sum_{\epsilon \in A} Z^*_{\delta,\epsilon} \tau^0_{\gamma,\epsilon,w} \tau^1_{\gamma,\epsilon,w} \quad (3r_D r_T^3) \quad (5056)$$

$$\tau^0_{\gamma,\delta,w} = \sum_{a \in V} {}^2D^1_{a,w} Y^3_{a,\gamma} Y^{1,*}_{a,\delta} \quad (3r_D r_T^2 N_v) \quad (5069)$$

$$\tau^3_{\gamma,\delta,w} = \sum_{\epsilon \in A} Z_{\epsilon,\gamma} \tau^2_{\epsilon,\delta,w} \quad (2r_D r_T^3) \quad (5057)$$

$$\tau^1_{\gamma,\alpha} = \sum_{a \in V} W^4_{a,\alpha} Y^1_{a,\gamma} \quad (2r_T r_V N_v) \quad (5070)$$

$$\tau^4_{\gamma,\delta,w} = \sum_{a \in V} {}^2D^1_{a,w} Y^3_{a,\gamma} Y^{1,*}_{a,\delta} \quad (3r_D r_T^2 N_v) \quad (5058)$$

$$\tau^2_{\gamma,\alpha} = \sum_{i \in O} W^3_{i,\alpha} Y^2_{i,\gamma} \quad (2r_T r_V N_o) \quad (5071)$$

$$\tau^5_{\gamma,\alpha} = \sum_{a \in V} W^4_{a,\alpha} Y^1_{a,\gamma} \quad (2r_T r_V N_v) \quad (5059)$$

$$\tau^3_{\gamma,\alpha} = \sum_{\beta \in B} X_{\alpha,\beta} \tau^1_{\gamma,\beta} \tau^2_{\gamma,\beta} \quad (3r_T r_V^2) \quad (5072)$$

$$\tau^6_{\gamma,\alpha} = \sum_{i \in O} W^3_{i,\alpha} Y^2_{i,\gamma} \quad (2r_T r_V N_o) \quad (5060)$$

$$\tau^4_{\gamma,\alpha} = \sum_{\delta \in A} Z_{\delta,\gamma} \tau^3_{\delta,\alpha} \quad (2r_T^2 r_V) \quad (5073)$$

$$\tau^5_{\gamma,\alpha} = \sum_{a \in V} W^2_{a,\alpha} Y^3_{a,\gamma} \quad (2r_T r_V N_v) \quad (5074)$$

$$\tau^3_{\gamma,\delta,w} = \sum_{\epsilon \in A} Z_{\epsilon,\gamma} \tau^2_{\epsilon,\delta,w} \quad (2r_D r_T^3) \quad (5087)$$

$$\tau^6_{\gamma,i} = \sum_{\alpha \in B} W^1_{i,\alpha} \tau^4_{\gamma,\alpha} \tau^5_{\gamma,\alpha} \quad (3r_T r_V N_o) \quad (5075)$$

$$\tau^4_{\gamma,\delta,w} = \sum_{a \in V} {}^2D^1_{a,w} Y^3_{a,\gamma} Y^{1,*}_{a,\delta} \quad (3r_D r_T^2 N_v) \quad (5088)$$

$$\tau^7_{i,j} = \sum_{\gamma \in A} Y^4_{j,\gamma} \tau^6_{\gamma,i} \quad (2r_T N_o^2) \quad (5076)$$

$$\tau^5_{\gamma,\alpha} = \sum_{a \in V} W^2_{a,\alpha} Y^1_{a,\gamma} \quad (2r_T r_V N_v) \quad (5089)$$

$$\tau^8_{\gamma,i} = \sum_{j \in O} Y^2_{j,\gamma} \tau^7_{j,i} \quad (2r_T N_o^2) \quad (5077)$$

$$\tau^6_{\gamma,\alpha} = \sum_{a \in V} W^4_{a,\alpha} Y^3_{a,\gamma} \quad (2r_T r_V N_v) \quad (5090)$$

$$\tau^9_{\gamma,\delta,w} = \sum_{i \in O} {}^2D^4_{i,w} Y^{4,*}_{i,\delta} \tau^8_{\gamma,i} \quad (3r_D r_T^2 N_o) \quad (5078)$$

$$\tau^7_{\gamma,\alpha} = \sum_{i \in O} W^3_{i,\alpha} Y^4_{i,\gamma} \quad (2r_T r_V N_o) \quad (5091)$$

$$\tau^{10}_{\gamma,\delta,w} = \sum_{a \in V} {}^2D^3_{a,w} Y^1_{a,\gamma} Y^{3,*}_{a,\delta} \quad (3r_D r_T^2 N_v) \quad (5079)$$

$$\tau^8_{\gamma,\alpha} = \sum_{\beta \in B} X_{\alpha,\beta} \tau^6_{\gamma,\beta} \tau^7_{\gamma,\beta} \quad (3r_T r_V^2) \quad (5092)$$

$$\tau^{11}_{\gamma,\delta,w} = \sum_{\epsilon \in A} Z^*_{\delta,\epsilon} \tau^{10}_{\gamma,\epsilon,w} \tau^9_{\gamma,\epsilon,w} \quad (3r_D r_T^3) \quad (5080)$$

$$\tau^9_{\gamma,\alpha} = \sum_{\delta \in A} Z_{\gamma,\delta} \tau^8_{\delta,\alpha} \quad (2r_T^2 r_V) \quad (5093)$$

$$\tau^{12}_{\gamma,\delta,w} = \sum_{\epsilon \in A} Z_{\epsilon,\gamma} \tau^{11}_{\epsilon,\delta,w} \quad (2r_D r_T^3) \quad (5081)$$

$$\tau^{10}_{\gamma,i} = \sum_{\alpha \in B} W^1_{i,\alpha} \tau^5_{\gamma,\alpha} \tau^9_{\gamma,\alpha} \quad (3r_T r_V N_o) \quad (5094)$$

$${}^2R^2_{i,\gamma} \leftarrow - \sum_{\delta \in A} \sum_{w \in D} \frac{1}{2} {}^2D^2_{i,w} Y^4_{i,\delta} \tau^0_{\delta,\gamma,w} \tau^{12}_{\delta,\gamma,w} \quad (4r_D r_T^2 N_o) \quad (5082)$$

$$\tau^{11}_{i,j} = \sum_{\gamma \in A} Y^2_{j,\gamma} \tau^{10}_{\gamma,i} \quad (2r_T N_o^2) \quad (5095)$$

Raw expression

$$\tau^{12}_{\gamma,i} = \sum_{j \in O} Y^4_{j,\gamma} \tau^{11}_{j,i} \quad (2r_T N_o^2) \quad (5096)$$

$${}^2R^2_{i,\epsilon} \leftarrow - \sum_{\gamma \in A} \sum_{j \in O} \sum_{k \in O} \sum_{l \in O} \sum_{a \in V} \sum_{b \in V} \sum_{c \in V} \sum_{d \in V} \frac{1}{2} \quad (5083)$$

$$Y^{1,*}_{a,\epsilon} \quad Z^*_{\epsilon,\gamma} \quad Y^{3,*}_{b,\gamma} \quad Y^{4,*}_{j,\gamma} \quad {}^2D^{a,i,b,j} \quad {}^2T_{b,k,d,l} \quad {}^2T_{c,j,a,i} \quad V_{k,c,l,d}$$

$${}^2R^2_{i,\gamma} \leftarrow - \sum_{\delta \in A} \sum_{w \in D} \frac{1}{2} {}^2D^2_{i,w} \tau^{12}_{\delta,i} \tau^3_{\delta,\gamma,w} \tau^4_{\delta,\gamma,w} \quad (4r_D r_T^2 N_o) \quad (5097)$$

Factorized expression

Raw expression

$$\tau^0_{\gamma,\delta,w} = \sum_{a \in V} {}^2D^3_{a,w} Y^1_{a,\gamma} Y^{3,*}_{a,\delta} \quad (3r_D r_T^2 N_v) \quad (5084)$$

$${}^2R^2_{i,\epsilon} \leftarrow - \sum_{\gamma \in A} \sum_{j \in O} \sum_{k \in O} \sum_{l \in O} \sum_{a \in V} \sum_{b \in V} \sum_{c \in V} \sum_{d \in V} \frac{1}{2} \quad (5098)$$

$$Y^{1,*}_{a,\epsilon} \quad Z^*_{\epsilon,\gamma} \quad Y^{3,*}_{b,\gamma} \quad Y^{4,*}_{j,\gamma} \quad {}^2D^{a,i,b,j} \quad {}^2T_{b,l,d,j} \quad {}^2T_{c,k,a,i} \quad V_{k,c,l,d}$$

$$\tau^1_{\gamma,\delta,w} = \sum_{i \in O} {}^2D^4_{i,w} Y^2_{i,\gamma} Y^{4,*}_{i,\delta} \quad (3r_D r_T^2 N_o) \quad (5085)$$

Factorized expression

$$\tau^2_{\gamma,\delta,w} = \sum_{\epsilon \in A} Z^*_{\delta,\epsilon} \tau^0_{\gamma,\epsilon,w} \tau^1_{\gamma,\epsilon,w} \quad (3r_D r_T^3) \quad (5086)$$

$$\tau^0_{\gamma,\delta,w} = \sum_{a \in V} {}^2D^1_{a,w} Y^3_{a,\gamma} Y^{1,*}_{a,\delta} \quad (3r_D r_T^2 N_v) \quad (5099)$$



$$\tau^1_{\gamma,\delta,w} = \sum_{a \in V} {}^2D^3_{a,w} Y^1_{a,\gamma} Y^{3,*}_{a,\delta} \quad (3r_D r_T^2 N_v) \quad (5100)$$

$$\tau^2_{\gamma,\delta,w} = \sum_{i \in O} {}^2D^4_{i,w} Y^2_{i,\gamma} Y^{4,*}_{i,\delta} \quad (3r_D r_T^2 N_o) \quad (5101)$$

$$\tau^3_{\gamma,\delta,w} = \sum_{\epsilon \in A} Z^*_{\delta,\epsilon} \tau^1_{\gamma,\epsilon,w} \tau^2_{\gamma,\epsilon,w} \quad (3r_D r_T^3) \quad (5102)$$

$$\tau^4_{\gamma,\alpha} = \sum_{a \in V} W^4_{a,\alpha} Y^3_{a,\gamma} \quad (2r_T r_V N_v) \quad (5103)$$

$$\tau^5_{\gamma,\alpha} = \sum_{i \in O} W^3_{i,\alpha} Y^4_{i,\gamma} \quad (2r_T r_V N_o) \quad (5104)$$

$$\tau^6_{\gamma,\alpha} = \sum_{\beta \in B} X_{\alpha,\beta} \tau^4_{\gamma,\beta} \tau^5_{\gamma,\beta} \quad (3r_T r_V^2) \quad (5105)$$

$$\tau^7_{\gamma,\alpha} = \sum_{\delta \in A} Z_{\gamma,\delta} \tau^6_{\delta,\alpha} \quad (2r_T^2 r_V) \quad (5106)$$

$$\tau^8_{\gamma,\alpha} = \sum_{a \in V} W^2_{a,\alpha} Y^1_{a,\gamma} \quad (2r_T r_V N_v) \quad (5107)$$

$$\tau^9_{\gamma,\delta,i} = \sum_{\alpha \in B} W^1_{i,\alpha} \tau^7_{\delta,\alpha} \tau^8_{\gamma,\alpha} \quad (3r_T^2 r_V N_o) \quad (5108)$$

$$\tau^{10}_{\gamma,\delta,\epsilon} = \sum_{i \in O} Z_{\gamma,\epsilon} Y^4_{i,\delta} \tau^9_{\gamma,\delta,i} \quad (3r_T^3 N_o) \quad (5109)$$

$$\tau^{11}_{\gamma,\delta,i} = \sum_{\epsilon \in A} Y^2_{i,\epsilon} \tau^{10}_{\epsilon,\gamma,\delta} \quad (2r_T^3 N_o) \quad (5110)$$

$$\tau^{12}_{\gamma,\delta,w,i} = \sum_{\epsilon \in A} \tau^{11}_{\epsilon,\gamma,i} \tau^3_{\epsilon,\delta,w} \quad (2r_D r_T^3 N_o) \quad (5111)$$

$$\tau^{13}_{\gamma,w,i} = \sum_{\delta \in A} \tau^0_{\delta,\gamma,w} \tau^{12}_{\delta,\gamma,w,i} \quad (2r_D r_T^2 N_o) \quad (5112)$$

$${}^2R^2_{i,\gamma} \leftarrow - \sum_{w \in D} \frac{1}{2} {}^2D^2_{i,w} \tau^{13}_{\gamma,w,i} \quad (2r_D r_T N_o) \quad (5113)$$

Raw expression

$${}^2R^2_{i,\epsilon} \leftarrow - \sum_{\gamma \in A} \sum_{j \in O} \sum_{k \in O} \sum_{l \in O} \sum_{a \in V} \sum_{b \in V} \sum_{c \in V} \sum_{d \in V} \frac{1}{2} \quad (5114)$$

$$Y^{1,*}_{a,\epsilon} Z^*_{\epsilon,\gamma} Y^{3,*}_{b,\gamma} Y^{4,*}_{j,\gamma} {}^2D^{a,i,b,j} {}^2T_{c,i,a,k} {}^2T_{d,l,b,j} V_{k,c,l,d}$$

Factorized expression

$$\tau^0_{\gamma,\delta,w} = \sum_{a \in V} {}^2D^1_{a,w} Y^3_{a,\gamma} Y^{1,*}_{a,\delta} \quad (3r_D r_T^2 N_v) \quad (5115)$$

$$\tau^1_{\gamma,\delta,w} = \sum_{a \in V} {}^2D^3_{a,w} Y^3_{a,\gamma} Y^{3,*}_{a,\delta} \quad (3r_D r_T^2 N_v) \quad (5116)$$

$$\tau^2_{\gamma,\delta,w} = \sum_{i \in O} {}^2D^4_{i,w} Y^4_{i,\gamma} Y^{4,*}_{i,\delta} \quad (3r_D r_T^2 N_o) \quad (5117)$$

$$\tau^3_{\gamma,\delta,w} = \sum_{\epsilon \in A} Z^*_{\delta,\epsilon} \tau^1_{\gamma,\epsilon,w} \tau^2_{\gamma,\epsilon,w} \quad (3r_D r_T^3) \quad (5118)$$

$$\tau^4_{\gamma,\alpha} = \sum_{a \in V} W^2_{a,\alpha} Y^1_{a,\gamma} \quad (2r_T r_V N_v) \quad (5119)$$

$$\tau^5_{\gamma,\alpha} = \sum_{a \in V} W^4_{a,\alpha} Y^1_{a,\gamma} \quad (2r_T r_V N_v) \quad (5120)$$

$$\tau^6_{\gamma,\alpha} = \sum_{i \in O} W^3_{i,\alpha} Y^2_{i,\gamma} \quad (2r_T r_V N_o) \quad (5121)$$

$$\tau^7_{\gamma,\alpha} = \sum_{\beta \in B} X_{\alpha,\beta} \tau^5_{\gamma,\beta} \tau^6_{\gamma,\beta} \quad (3r_T r_V^2) \quad (5122)$$

$$\tau^8_{\gamma,\alpha} = \sum_{\delta \in A} Z_{\delta,\gamma} \tau^7_{\delta,\alpha} \quad (2r_T^2 r_V) \quad (5123)$$

$$\tau^9_{\gamma,\delta,i} = \sum_{\alpha \in B} W^1_{i,\alpha} \tau^4_{\gamma,\alpha} \tau^8_{\delta,\alpha} \quad (3r_T^2 r_V N_o) \quad (5124)$$

$$\tau^{10}_{\gamma,\delta,\epsilon} = \sum_{i \in O} Z_{\gamma,\delta} Y^4_{i,\delta} \tau^9_{\gamma,\epsilon,i} \quad (3r_T^3 N_o) \quad (5125)$$

$$\tau^{11}_{\gamma,\delta,i} = \sum_{\epsilon \in A} Y^2_{i,\epsilon} \tau^{10}_{\epsilon,\gamma,\delta} \quad (2r_T^3 N_o) \quad (5126)$$

$$\tau^{12}_{\gamma,\delta,w,i} = \sum_{\epsilon \in A} \tau^{11}_{\gamma,\epsilon,i} \tau^3_{\epsilon,\delta,w} \quad (2r_D r_T^3 N_o) \quad (5127)$$

$$\tau_{\gamma,w,i}^{13} = \sum_{\delta \in A} \tau_{\delta,\gamma,w}^0 \tau_{\delta,\gamma,w,i}^{12} \quad (2r_D r_T^2 N_o) \quad (5128)$$

$$\tau_{\gamma,\delta,w}^{10} = \sum_{i \in O} {}^2D_{i,w}^4 Y_{i,\gamma}^4 Y_{i,\delta}^{4,*} \quad (3r_D r_T^2 N_o) \quad (5141)$$

$${}^2R_{i,\gamma}^2 \leftarrow - \sum_{w \in D} \frac{1}{2} {}^2D_{i,w}^2 \tau_{\gamma,w,i}^{13} \quad (2r_D r_T N_o) \quad (5129)$$

$$\tau_{\gamma,\delta,w}^{11} = \sum_{\epsilon \in A} Z_{\delta,\epsilon}^* \tau_{\gamma,\epsilon,w}^{10} \tau_{\gamma,\epsilon,w}^9 \quad (3r_D r_T^3) \quad (5142)$$

Raw expression

$$\tau_{\gamma,\delta,w}^{12} = \sum_{\epsilon \in A} Z_{\gamma,\epsilon} \tau_{\epsilon,\delta,w}^{11} \quad (2r_D r_T^3) \quad (5143)$$

$${}^2R_{i,\epsilon}^2 \leftarrow - \sum_{\gamma \in A} \sum_{j \in O} \sum_{k \in O} \sum_{l \in O} \sum_{a \in V} \sum_{b \in V} \sum_{c \in V} \sum_{d \in V} \frac{1}{2} \quad (5130)$$

$$Y_{a,\epsilon}^{1,*} Z_{\epsilon,\gamma}^* Y_{b,\gamma}^{3,*} Y_{j,\gamma}^{4,*} {}^2D_{a,i,b,j} {}^2T_{c,i,b,j} {}^2T_{d,k,a,l} V_{k,d,l,c}$$

$${}^2R_{i,\gamma}^2 \leftarrow - \sum_{\delta \in A} \sum_{w \in D} \frac{1}{2} {}^2D_{i,w}^2 Y_{i,\delta}^2 \tau_{\delta,\gamma,w}^{12} \tau_{\delta,\gamma,w}^8 \quad (4r_D r_T^2 N_o) \quad (5144)$$

Factorized expression

Raw expression

$$\tau_{\gamma,\alpha}^0 = \sum_{a \in V} W_{a,\alpha}^2 Y_{a,\gamma}^1 \quad (2r_T r_V N_v) \quad (5131)$$

$${}^2R_{i,\epsilon}^2 \leftarrow - \sum_{\gamma \in A} \sum_{j \in O} \sum_{k \in O} \sum_{l \in O} \sum_{a \in V} \sum_{b \in V} \sum_{c \in V} \sum_{d \in V} \frac{1}{2} \quad (5145)$$

$$Y_{a,\epsilon}^{1,*} Z_{\epsilon,\gamma}^* Y_{b,\gamma}^{3,*} Y_{j,\gamma}^{4,*} {}^2D_{a,i,b,j} {}^2T_{c,j,a,i} {}^2T_{d,k,b,l} V_{k,d,l,c}$$

$$\tau_{\gamma,\alpha}^1 = \sum_{i \in O} W_{i,\alpha}^1 Y_{i,\gamma}^2 \quad (2r_T r_V N_o) \quad (5132)$$

Factorized expression

$$\tau_{\gamma,\alpha}^2 = \sum_{\beta \in B} X_{\beta,\alpha} \tau_{\gamma,\beta}^0 \tau_{\gamma,\beta}^1 \quad (3r_T r_V^2) \quad (5133)$$

$$\tau_{\gamma,\delta,w}^0 = \sum_{a \in V} {}^2D_{a,w}^1 Y_{a,\gamma}^3 Y_{a,\delta}^{1,*} \quad (3r_D r_T^2 N_v) \quad (5146)$$

$$\tau_{\gamma,\alpha}^3 = \sum_{\delta \in A} Z_{\delta,\gamma} \tau_{\delta,\alpha}^2 \quad (2r_T^2 r_V) \quad (5134)$$

$$\tau_{\gamma,\delta,w}^1 = \sum_{a \in V} {}^2D_{a,w}^3 Y_{a,\gamma}^3 Y_{a,\delta}^{3,*} \quad (3r_D r_T^2 N_v) \quad (5147)$$

$$\tau_{\gamma,\alpha}^4 = \sum_{i \in O} W_{i,\alpha}^3 Y_{i,\gamma}^4 \quad (2r_T r_V N_o) \quad (5135)$$

$$\tau_{\gamma,\alpha}^2 = \sum_{a \in V} W_{a,\alpha}^2 Y_{a,\gamma}^1 \quad (2r_T r_V N_v) \quad (5148)$$

$$\tau_{\gamma,a}^5 = \sum_{\alpha \in B} W_{a,\alpha}^4 \tau_{\gamma,\alpha}^3 \tau_{\gamma,\alpha}^4 \quad (3r_T r_V N_v) \quad (5136)$$

$$\tau_{\gamma,\alpha}^3 = \sum_{i \in O} W_{i,\alpha}^1 Y_{i,\gamma}^2 \quad (2r_T r_V N_o) \quad (5149)$$

$$\tau_{\gamma,\delta}^6 = \sum_{a \in V} Y_{a,\gamma}^1 \tau_{\delta,a}^5 \quad (2r_T^2 N_v) \quad (5137)$$

$$\tau_{\gamma,\alpha}^4 = \sum_{\beta \in B} X_{\beta,\alpha} \tau_{\gamma,\beta}^2 \tau_{\gamma,\beta}^3 \quad (3r_T r_V^2) \quad (5150)$$

$$\tau_{\gamma,a}^7 = \sum_{\delta \in A} Y_{a,\delta}^3 \tau_{\gamma,\delta}^6 \quad (2r_T^2 N_v) \quad (5138)$$

$$\tau_{\gamma,\alpha}^5 = \sum_{\delta \in A} Z_{\delta,\gamma} \tau_{\delta,\alpha}^4 \quad (2r_T^2 r_V) \quad (5151)$$

$$\tau_{\gamma,\delta,w}^8 = \sum_{a \in V} {}^2D_{a,w}^1 Y_{a,\gamma}^{1,*} {}^2\tau_{\gamma,a}^7 \quad (3r_D r_T^2 N_v) \quad (5139)$$

$$\tau_{\gamma,\alpha}^6 = \sum_{a \in V} W_{a,\alpha}^4 Y_{a,\gamma}^1 \quad (2r_T r_V N_v) \quad (5152)$$

$$\tau_{\gamma,\delta,w}^9 = \sum_{a \in V} {}^2D_{a,w}^3 Y_{a,\gamma}^3 Y_{a,\delta}^{3,*} \quad (3r_D r_T^2 N_v) \quad (5140)$$

$$\tau_{\gamma,\delta,i}^7 = \sum_{\alpha \in B} W_{i,\alpha}^3 \tau_{\delta,\alpha}^5 \tau_{\gamma,\alpha}^6 \quad (3r_T^2 r_V N_o) \quad (5153)$$

$$\tau_{\gamma,\delta,\epsilon}^8 = \sum_{i \in O} Z_{\gamma,\delta} Y_{i,\delta}^4 \tau_{\gamma,\epsilon,i}^7 \quad (3r_T^3 N_o) \quad (5154)$$

$$\tau_{\gamma,a}^7 = \sum_{\alpha \in B} W_{a,\alpha}^4 \tau_{\gamma,\alpha}^5 \tau_{\gamma,\alpha}^6 \quad (3r_T r_V N_v) \quad (5167)$$

$$\tau_{\gamma,\delta,i}^9 = \sum_{\epsilon \in A} Y_{i,\epsilon}^2 \tau_{\epsilon,\gamma,\delta}^8 \quad (2r_T^3 N_o) \quad (5155)$$

$$\tau_{\gamma,\delta}^8 = \sum_{a \in V} Y_{a,\gamma}^1 \tau_{\delta,a}^7 \quad (2r_T^2 N_v) \quad (5168)$$

$$\tau_{\gamma,\delta,w}^{10} = \sum_{\epsilon \in A} \sum_{i \in O} {}^2D_{i,w}^4 Y_{i,\delta}^{4,*} \tau_{\epsilon,\delta,w}^1 \tau_{\epsilon,\gamma,i}^9 \quad (4r_D r_T^3 N_o) \quad (5156)$$

$$\tau_{\gamma,a}^9 = \sum_{\delta \in A} Y_{a,\delta}^3 \tau_{\gamma,\delta}^8 \quad (2r_T^2 N_v) \quad (5169)$$

$$\tau_{\gamma,\delta,w}^{11} = \sum_{\epsilon \in A} Z_{\delta,\epsilon}^* \tau_{\gamma,\epsilon,w}^{10} \quad (2r_D r_T^3) \quad (5157)$$

$$\tau_{\gamma,\delta,w}^{10} = \sum_{a \in V} {}^2D_{a,w}^3 Y_{a,\delta}^{3,*} \tau_{\gamma,a}^9 \quad (3r_D r_T^2 N_v) \quad (5170)$$

$${}^2R_{i,\gamma}^2 \leftarrow - \sum_{\delta \in A} \sum_{w \in D} \frac{1}{2} {}^2D_{i,w}^2 Y_{i,\delta}^4 \tau_{\delta,\gamma,w}^0 \tau_{\delta,\gamma,w}^{11} \quad (4r_D r_T^2 N_o) \quad (5158)$$

Raw expression

$$\tau_{\gamma,\delta,w}^{12} = \sum_{\epsilon \in A} Z_{\epsilon,\gamma} \tau_{\epsilon,\delta,w}^{11} \quad (2r_D r_T^3) \quad (5172)$$

$${}^2R_{i,\epsilon}^2 \leftarrow - \sum_{\gamma \in A} \sum_{j \in O} \sum_{k \in O} \sum_{l \in O} \sum_{a \in V} \sum_{b \in V} \sum_{c \in V} \sum_{d \in V} \frac{1}{2} \quad (5159)$$

$$Y_{a,\epsilon}^{1,*} Z_{\epsilon,\gamma}^* Y_{b,\gamma}^{3,*} Y_{j,\gamma}^{4,*} {}^2D_{a,i,b,j} {}^2T_{c,k,a,i} {}^2T_{d,j,b,l} V_{k,c,l,d}$$

$${}^2R_{i,\gamma}^2 \leftarrow - \sum_{\delta \in A} \sum_{w \in D} \frac{1}{2} {}^2D_{i,w}^2 Y_{i,\delta}^4 \tau_{\delta,\gamma,w}^0 \tau_{\delta,\gamma,w}^{12} \quad (4r_D r_T^2 N_o) \quad (5173)$$

Factorized expression

Raw expression

$$\tau_{\gamma,\delta,w}^0 = \sum_{a \in V} {}^2D_{a,w}^1 Y_{a,\gamma}^3 Y_{a,\delta}^{1,*} \quad (3r_D r_T^2 N_v) \quad (5160)$$

$${}^2R_{i,\epsilon}^2 \leftarrow - \sum_{\gamma \in A} \sum_{j \in O} \sum_{k \in O} \sum_{l \in O} \sum_{a \in V} \sum_{b \in V} \sum_{c \in V} \sum_{d \in V} \frac{1}{2} \quad (5174)$$

$$Y_{a,\epsilon}^{1,*} Z_{\epsilon,\gamma}^* Y_{b,\gamma}^{3,*} Y_{j,\gamma}^{4,*} {}^2D_{a,i,b,j} {}^2T_{c,k,a,i} {}^2T_{d,l,b,j} V_{k,d,l,c}$$

$$\tau_{\gamma,\delta,w}^1 = \sum_{i \in O} {}^2D_{i,w}^4 Y_{i,\gamma}^2 Y_{i,\delta}^{4,*} \quad (3r_D r_T^2 N_o) \quad (5161)$$

Factorized expression

$$\tau_{\gamma,\alpha}^2 = \sum_{a \in V} W_{a,\alpha}^2 Y_{a,\gamma}^1 \quad (2r_T r_V N_v) \quad (5162)$$

$$\tau_{\gamma,\delta,w}^0 = \sum_{a \in V} {}^2D_{a,w}^1 Y_{a,\gamma}^3 Y_{a,\delta}^{1,*} \quad (3r_D r_T^2 N_v) \quad (5175)$$

$$\tau_{\gamma,\alpha}^3 = \sum_{i \in O} W_{i,\alpha}^1 Y_{i,\gamma}^2 \quad (2r_T r_V N_o) \quad (5163)$$

$$\tau_{\gamma,\delta,w}^1 = \sum_{a \in V} {}^2D_{a,w}^3 Y_{a,\gamma}^3 Y_{a,\delta}^{3,*} \quad (3r_D r_T^2 N_v) \quad (5176)$$

$$\tau_{\gamma,\alpha}^4 = \sum_{\beta \in B} X_{\beta,\alpha} \tau_{\gamma,\beta}^2 \tau_{\gamma,\beta}^3 \quad (3r_T r_V^2) \quad (5164)$$

$$\tau_{\gamma,\delta,w}^2 = \sum_{i \in O} {}^2D_{i,w}^4 Y_{i,\gamma}^4 Y_{i,\delta}^{4,*} \quad (3r_D r_T^2 N_o) \quad (5177)$$

$$\tau_{\gamma,\alpha}^5 = \sum_{\delta \in A} Z_{\delta,\gamma} \tau_{\delta,\alpha}^4 \quad (2r_T^2 r_V) \quad (5165)$$

$$\tau_{\gamma,\delta,w}^3 = \sum_{\epsilon \in A} Z_{\delta,\epsilon}^* \tau_{\gamma,\epsilon,w}^1 \tau_{\gamma,\epsilon,w}^2 \quad (3r_D r_T^3) \quad (5178)$$

$$\tau_{\gamma,\alpha}^6 = \sum_{i \in O} W_{i,\alpha}^3 Y_{i,\gamma}^4 \quad (2r_T r_V N_o) \quad (5166)$$

$$\tau_{\gamma,\alpha}^4 = \sum_{a \in V} W_{a,\alpha}^2 Y_{a,\gamma}^1 \quad (2r_T r_V N_v) \quad (5179)$$

$$\tau^5_{\gamma,\alpha,i} = \sum_{\beta \in B} W^1_{i,\beta} X_{\beta,\alpha} \tau^4_{\gamma,\beta} \quad (3r_T r_V^2 N_o) \quad (5180)$$

$$\tau^3_{\gamma,\alpha} = \sum_{i \in O} W^3_{i,\alpha} Y^4_{i,\gamma} \quad (2r_T r_V N_o) \quad (5193)$$

$$\tau^6_{\gamma,\alpha} = \sum_{i \in O} W^3_{i,\alpha} Y^2_{i,\gamma} \quad (2r_T r_V N_o) \quad (5181)$$

$$\tau^4_{\gamma,\alpha} = \sum_{\delta \in A} \sum_{i \in O} Y^2_{i,\gamma} Z_{\gamma,\delta} \tau^3_{\delta,\alpha} \tau^2_{\delta,\alpha,i} \quad (4r_T^2 r_V N_o) \quad (5194)$$

$$\tau^7_{\gamma,\alpha} = \sum_{a \in V} W^4_{a,\alpha} Y^1_{a,\gamma} \quad (2r_T r_V N_v) \quad (5182)$$

$$\tau^5_{\gamma,a} = \sum_{\alpha \in B} W^4_{a,\alpha} \tau^4_{\gamma,\alpha} \quad (2r_T r_V N_v) \quad (5195)$$

$$\tau^8_{\gamma,\delta,i} = \sum_{\alpha \in B} \tau^6_{\gamma,\alpha} \tau^7_{\delta,\alpha} \tau^5_{\gamma,\alpha,i} \quad (3r_T^2 r_V N_o) \quad (5183)$$

$$\tau^6_{\gamma,\delta} = \sum_{a \in V} Y^3_{a,\delta} \tau^5_{\gamma,a} \quad (2r_T^2 N_v) \quad (5196)$$

$$\tau^9_{\gamma,\delta} = \sum_{i \in O} Y^2_{i,\delta} \tau^8_{\gamma,\delta,i} \quad (2r_T^2 N_o) \quad (5184)$$

$$\tau^7_{\gamma,a} = \sum_{\delta \in A} Y^1_{a,\delta} \tau^6_{\delta,\gamma} \quad (2r_T^2 N_v) \quad (5197)$$

$$\tau^{10}_{\gamma,\delta} = \sum_{\epsilon \in A} Z_{\epsilon,\delta} \tau^9_{\gamma,\epsilon} \quad (2r_T^3) \quad (5185)$$

$$\tau^8_{\gamma,\delta,w} = \sum_{a \in V} {}^2D^3_{a,w} Y^{3,*}_{a,\delta} \tau^7_{\gamma,a} \quad (3r_D r_T^2 N_v) \quad (5198)$$

$$\tau^{11}_{\gamma,\delta} = \sum_{\epsilon \in A} Z_{\epsilon,\gamma} \tau^{10}_{\epsilon,\delta} \quad (2r_T^3) \quad (5186)$$

$$\tau^9_{\gamma,\delta,w} = \sum_{i \in O} {}^2D^4_{i,w} Y^4_{i,\gamma} Y^{4,*}_{i,\delta} \quad (3r_D r_T^2 N_o) \quad (5199)$$

$$\tau^{12}_{\gamma,\delta,w} = \sum_{\epsilon \in A} \tau^{11}_{\epsilon,\gamma} \tau^3_{\epsilon,\delta,w} \quad (2r_D r_T^3) \quad (5187)$$

$$\tau^{10}_{\gamma,\delta,w} = \sum_{\epsilon \in A} Z^*_{\delta,\epsilon} \tau^8_{\gamma,\epsilon,w} \tau^9_{\gamma,\epsilon,w} \quad (3r_D r_T^3) \quad (5200)$$

$${}^2R^2_{i,\gamma} \leftarrow - \sum_{\delta \in A} \sum_{w \in D} \frac{1}{2} {}^2D^2_{i,w} Y^4_{i,\delta} \tau^0_{\delta,\gamma,w} \tau^{12}_{\delta,\gamma,w} \quad (4r_D r_T^2 N_o) \quad (5188)$$

$$\tau^{11}_{\gamma,\delta,w} = \sum_{\epsilon \in A} Z_{\gamma,\epsilon} \tau^{10}_{\epsilon,\delta,w} \quad (2r_D r_T^3) \quad (5201)$$

Raw expression

$${}^2R^2_{i,\epsilon} \leftarrow \sum_{\gamma \in A} \sum_{j \in O} \sum_{k \in O} \sum_{l \in O} \sum_{a \in V} \sum_{b \in V} \sum_{c \in V} \sum_{d \in V} \frac{1}{4} Y^{1,*}_{a,\epsilon} Z^*_{\epsilon,\gamma} Y^{3,*}_{b,\gamma} Y^{4,*}_{j,\gamma} {}^2D^{a,i,b,j} {}^2T_{a,i,b,k} {}^2T_{c,j,d,l} V_{k,d,l,c} \quad (5189)$$

Factorized expression

$$\tau^0_{\gamma,\delta,w} = \sum_{a \in V} {}^2D^1_{a,w} Y^1_{a,\gamma} Y^{1,*}_{a,\delta} \quad (3r_D r_T^2 N_v) \quad (5190)$$

$${}^2R^2_{i,\gamma} \leftarrow \sum_{\delta \in A} \sum_{w \in D} \frac{1}{4} {}^2D^2_{i,w} Y^2_{i,\delta} \tau^0_{\delta,\gamma,w} \tau^{11}_{\delta,\gamma,w} \quad (4r_D r_T^2 N_o) \quad (5202)$$

Raw expression

$${}^2R^2_{i,\epsilon} \leftarrow \sum_{\gamma \in A} \sum_{j \in O} \sum_{k \in O} \sum_{l \in O} \sum_{a \in V} \sum_{b \in V} \sum_{c \in V} \sum_{d \in V} \frac{1}{4} Y^{1,*}_{a,\epsilon} Z^*_{\epsilon,\gamma} Y^{3,*}_{b,\gamma} Y^{4,*}_{j,\gamma} {}^2D^{a,i,b,j} {}^2T_{a,i,b,k} {}^2T_{c,l,d,j} V_{k,c,l,d} \quad (5203)$$

Factorized expression

$$\tau^0_{\gamma,\delta,w} = \sum_{a \in V} {}^2D^1_{a,w} Y^1_{a,\gamma} Y^{1,*}_{a,\delta} \quad (3r_D r_T^2 N_v) \quad (5204)$$

$$\tau^2_{\gamma,\alpha,i} = \sum_{\beta \in B} W^1_{i,\beta} X_{\beta,\alpha} \tau^1_{\gamma,\beta} \quad (3r_T r_V^2 N_o) \quad (5192)$$

$$\tau^1_{\gamma,\delta,w} = \sum_{a \in V} {}^2D^3_{a,w} Y^1_{a,\gamma} Y^{3,*}_{a,\delta} \quad (3r_D r_T^2 N_v) \quad (5205)$$

$$\tau^2_{\gamma,\alpha} = \sum_{a \in V} W^4_{a,\alpha} Y^3_{a,\gamma} \quad (2r_T r_V N_v) \quad (5206)$$

$$\tau^3_{\gamma,\alpha,i} = \sum_{\beta \in B} X_{\alpha,\beta} W^3_{i,\beta} \tau^2_{\gamma,\beta} \quad (3r_T r_V^2 N_o) \quad (5207)$$

$$\tau^4_{\gamma,\alpha} = \sum_{i \in O} W^1_{i,\alpha} Y^4_{i,\gamma} \quad (2r_T r_V N_o) \quad (5208)$$

$$\tau^5_{\gamma,\alpha} = \sum_{a \in V} W^2_{a,\alpha} Y^3_{a,\gamma} \quad (2r_T r_V N_v) \quad (5209)$$

$$\tau^6_{\gamma,\delta,i} = \sum_{\alpha \in B} \tau^4_{\gamma,\alpha} \tau^5_{\delta,\alpha} \tau^3_{\gamma,\alpha,i} \quad (3r_T^2 r_V N_o) \quad (5210)$$

$$\tau^7_{\gamma,\delta,\epsilon} = \sum_{i \in O} Y^2_{i,\gamma} Z_{\gamma,\delta} \tau^6_{\epsilon,\delta,i} \quad (3r_T^3 N_o) \quad (5211)$$

$$\tau^8_{\gamma,\delta,i} = \sum_{\epsilon \in A} Y^4_{i,\epsilon} \tau^7_{\gamma,\epsilon,\delta} \quad (2r_T^3 N_o) \quad (5212)$$

$$\tau^9_{\gamma,\delta,w} = \sum_{\epsilon \in A} \sum_{i \in O} {}^2D^4_{i,w} Y^{4,*}_{i,\delta} \tau^1_{\epsilon,\delta,w} \tau^8_{\epsilon,\gamma,i} \quad (4r_D r_T^3 N_o) \quad (5213)$$

$$\tau^{10}_{\gamma,\delta,w} = \sum_{\epsilon \in A} Z^*_{\delta,\epsilon} \tau^9_{\gamma,\epsilon,w} \quad (2r_D r_T^3) \quad (5214)$$

$$\tau^{11}_{\gamma,\delta,w} = \sum_{\epsilon \in A} Z_{\gamma,\epsilon} \tau^{10}_{\epsilon,\delta,w} \quad (2r_D r_T^3) \quad (5215)$$

$${}^2R^2_{i,\gamma} \leftarrow \sum_{\delta \in A} \sum_{w \in D} \frac{1}{4} {}^2D^2_{i,w} Y^2_{i,\delta} \tau^0_{\delta,\gamma,w} \tau^{11}_{\delta,\gamma,w} \quad (4r_D r_T^2 N_o) \quad (5216)$$

Raw expression

$${}^2R^2_{i,\epsilon} \leftarrow \sum_{\gamma \in A} \sum_{j \in O} \sum_{k \in O} \sum_{l \in O} \sum_{a \in V} \sum_{b \in V} \sum_{c \in V} \sum_{d \in V} \frac{1}{4} Y^{1,*}_{a,\epsilon} Z^*_{\epsilon,\gamma} Y^{3,*}_{b,\gamma} Y^{4,*}_{j,\gamma} {}^2D^{a,i,b,j} {}^2T_{a,i,c,j} {}^2T_{b,k,d,l} V_{k,d,l,c} \quad (5217)$$

Factorized expression

$$\tau^0_{\gamma,\delta,w} = \sum_{a \in V} {}^2D^1_{a,w} Y^1_{a,\gamma} Y^{1,*}_{a,\delta} \quad (3r_D r_T^2 N_v) \quad (5218)$$

$$\tau^1_{\gamma,\alpha} = \sum_{i \in O} W^1_{i,\alpha} Y^2_{i,\gamma} \quad (2r_T r_V N_o) \quad (5219)$$

$$\tau^2_{\gamma,\alpha} = \sum_{a \in V} W^2_{a,\alpha} Y^3_{a,\gamma} \quad (2r_T r_V N_v) \quad (5220)$$

$$\tau^3_{\gamma,\alpha,i} = \sum_{\delta \in A} Z_{\gamma,\delta} Y^4_{i,\delta} \tau^2_{\delta,\alpha} \quad (3r_T^2 r_V N_o) \quad (5221)$$

$$\tau^4_{\gamma,\delta,w} = \sum_{a \in V} {}^2D^3_{a,w} Y^1_{a,\gamma} Y^{3,*}_{a,\delta} \quad (3r_D r_T^2 N_v) \quad (5222)$$

$$\tau^5_{\gamma,\alpha} = \sum_{i \in O} W^3_{i,\alpha} Y^2_{i,\gamma} \quad (2r_T r_V N_o) \quad (5223)$$

$$\tau^6_{\gamma,\alpha} = \sum_{a \in V} W^4_{a,\alpha} Y^3_{a,\gamma} \quad (2r_T r_V N_v) \quad (5224)$$

$$\tau^7_{\gamma,\alpha,i} = \sum_{\delta \in A} Z_{\gamma,\delta} Y^4_{i,\delta} \tau^6_{\delta,\alpha} \quad (3r_T^2 r_V N_o) \quad (5225)$$

$$\tau^8_{\gamma,\alpha,w} = \sum_{\delta \in A} \sum_{i \in O} {}^2D^4_{i,w} Y^{4,*}_{i,\gamma} \tau^5_{\delta,\alpha} \tau^4_{\delta,\gamma,w} \tau^7_{\delta,\alpha,i} \quad (5r_D r_T^2 r_V N_o) \quad (5226)$$

$$\tau^9_{\gamma,\alpha,w} = \sum_{\beta \in B} X_{\alpha,\beta} \tau^8_{\gamma,\beta,w} \quad (2r_D r_T r_V^2) \quad (5227)$$

$$\tau^{10}_{\gamma,\alpha,w} = \sum_{\delta \in A} Z^*_{\gamma,\delta} \tau^9_{\delta,\alpha,w} \quad (2r_D r_T^2 r_V) \quad (5228)$$

$$\tau^{11}_{\gamma,\delta,w,i} = \sum_{\alpha \in B} \tau^1_{\gamma,\alpha} \tau^{10}_{\delta,\alpha,w} \tau^3_{\gamma,\alpha,i} \quad (3r_D r_T^2 r_V N_o) \quad (5229)$$

$$\tau^{12}_{\gamma,w,i} = \sum_{\delta \in A} \tau^0_{\delta,\gamma,w} \tau^{11}_{\delta,\gamma,w,i} \quad (2r_D r_T^2 N_o) \quad (5230)$$

$${}^2R^2_{i,\gamma} \leftarrow \sum_{w \in D} \frac{1}{4} {}^2D^2_{i,w} \tau^{12}_{\gamma,w,i} \quad (2r_D r_T N_o) \quad (5231)$$

Raw expression

$${}^2R^2_{i,\epsilon} \leftarrow \sum_{\gamma \in A} \sum_{j \in O} \sum_{k \in O} \sum_{l \in O} \sum_{a \in V} \sum_{b \in V} \sum_{c \in V} \sum_{d \in V} \frac{1}{4} Y^{1,*}_{a,\epsilon} Z^*_{\epsilon,\gamma} Y^{3,*}_{b,\gamma} Y^{4,*}_{j,\gamma} {}^2D^{a,i,b,j} {}^2T_{a,i,c,j} {}^2T_{d,k,b,l} V_{k,c,l,d} \quad (5232)$$

Factorized expression

$$\tau^0_{\gamma,\delta,w} = \sum_{a \in V} {}^2D^1_{a,w} Y^1_{a,\gamma} Y^{1,*}_{a,\delta} \quad (3r_D r_T^2 N_v) \quad (5233)$$

$$\tau^1_{\gamma,\delta,w} = \sum_{a \in V} {}^2D^3_{a,w} Y^3_{a,\gamma} Y^{3,*}_{a,\delta} \quad (3r_D r_T^2 N_v) \quad (5234)$$

$$\tau^2_{\gamma,\alpha} = \sum_{a \in V} W^4_{a,\alpha} Y^3_{a,\gamma} \quad (2r_T r_V N_v) \quad (5235)$$

$$\tau^3_{\gamma,\alpha,i} = \sum_{\beta \in B} X_{\alpha,\beta} W^3_{i,\beta} \tau^2_{\gamma,\beta} \quad (3r_T r_V^2 N_o) \quad (5236)$$

$$\tau^4_{\gamma,\alpha} = \sum_{i \in O} W^1_{i,\alpha} Y^4_{i,\gamma} \quad (2r_T r_V N_o) \quad (5237)$$

$$\tau^5_{\gamma,\alpha} = \sum_{a \in V} W^2_{a,\alpha} Y^1_{a,\gamma} \quad (2r_T r_V N_v) \quad (5238)$$

$$\tau^6_{\gamma,\delta,i} = \sum_{\alpha \in B} \tau^4_{\delta,\alpha} \tau^5_{\gamma,\alpha} \tau^3_{\delta,\alpha,i} \quad (3r_T^2 r_V N_o) \quad (5239)$$

$$\tau^7_{\gamma,\delta,\epsilon} = \sum_{i \in O} Z_{\gamma,\delta} Y^4_{i,\delta} \tau^6_{\gamma,\epsilon,i} \quad (3r_T^3 N_o) \quad (5240)$$

$$\tau^8_{\gamma,\delta,i} = \sum_{\epsilon \in A} Y^2_{i,\epsilon} \tau^7_{\epsilon,\gamma,\delta} \quad (2r_T^3 N_o) \quad (5241)$$

$$\tau^9_{\gamma,\delta,w} = \sum_{\epsilon \in A} \sum_{i \in O} {}^2D^4_{i,w} Y^{4,*}_{i,\delta} \tau^1_{\epsilon,\delta,w} \tau^8_{\epsilon,\gamma,i} \quad (4r_D r_T^3 N_o) \quad (5242)$$

$$\tau^{10}_{\gamma,\delta,w} = \sum_{\epsilon \in A} Z^*_{\delta,\epsilon} \tau^9_{\gamma,\epsilon,w} \quad (2r_D r_T^3) \quad (5243)$$

$$\tau^{11}_{\gamma,\delta,w} = \sum_{\epsilon \in A} Z_{\gamma,\epsilon} \tau^{10}_{\epsilon,\delta,w} \quad (2r_D r_T^3) \quad (5244)$$

$${}^2R^2_{i,\gamma} \leftarrow \sum_{\delta \in A} \sum_{w \in D} \frac{1}{4} {}^2D^2_{i,w} Y^2_{i,\delta} \tau^0_{\delta,\gamma,w} \tau^{11}_{\delta,\gamma,w} \quad (4r_D r_T^2 N_o) \quad (5245)$$

Raw expression

$${}^2R^2_{i,\epsilon} \leftarrow \sum_{\gamma \in A} \sum_{j \in O} \sum_{k \in O} \sum_{l \in O} \sum_{a \in V} \sum_{b \in V} \sum_{c \in V} \sum_{d \in V} \frac{1}{4} Y^{1,*}_{a,\epsilon} Z^*_{\epsilon,\gamma} Y^{3,*}_{b,\gamma} Y^{4,*}_{j,\gamma} {}^2D^{a,i,b,j} {}^2T_{a,i,c,k} {}^2T_{b,l,d,j} V_{k,d,l,c} \quad (5246)$$

Factorized expression

$$\tau^0_{\gamma,\delta,w} = \sum_{a \in V} {}^2D^1_{a,w} Y^1_{a,\gamma} Y^{1,*}_{a,\delta} \quad (3r_D r_T^2 N_v) \quad (5247)$$

$$\tau^1_{\gamma,\delta,w} = \sum_{a \in V} {}^2D^3_{a,w} Y^3_{a,\gamma} Y^{3,*}_{a,\delta} \quad (3r_D r_T^2 N_v) \quad (5248)$$

$$\tau^2_{\gamma,\alpha} = \sum_{a \in V} W^2_{a,\alpha} Y^1_{a,\gamma} \quad (2r_T r_V N_v) \quad (5249)$$

$$\tau^3_{\gamma,\alpha,i} = \sum_{\beta \in B} W^1_{i,\beta} X_{\beta,\alpha} \tau^2_{\gamma,\beta} \quad (3r_T r_V^2 N_o) \quad (5250)$$

$$\tau^4_{\gamma,\alpha} = \sum_{i \in O} W^3_{i,\alpha} Y^2_{i,\gamma} \quad (2r_T r_V N_o) \quad (5251)$$

$$\tau^5_{\gamma,\alpha} = \sum_{a \in V} W^4_{a,\alpha} Y^3_{a,\gamma} \quad (2r_T r_V N_v) \quad (5252)$$

$$\tau^6_{\gamma,\delta,i} = \sum_{\alpha \in B} \tau^4_{\gamma,\alpha} \tau^5_{\delta,\alpha} \tau^3_{\gamma,\alpha,i} \quad (3r_T^2 r_V N_o) \quad (5253)$$

$$\tau^7_{\gamma,i} = \sum_{\delta \in A} Z_{\delta,\gamma} \tau^6_{\delta,\gamma,i} \quad (2r_T^2 N_o) \quad (5254)$$

$$\tau^8_{i,j} = \sum_{\gamma \in A} Y^4_{j,\gamma} \tau^7_{\gamma,i} \quad (2r_T N_o^2) \quad (5255)$$

$$\tau^9_{\gamma,i} = \sum_{j \in O} Y^4_{j,\gamma} \tau^8_{j,i} \quad (2r_T N_o^2) \quad (5256)$$

$$\tau^{10}_{\gamma,\delta,w} = \sum_{i \in O} {}^2D^4_{i,w} Y^{4,*}_{i,\delta} \tau^9_{\gamma,i} \quad (3r_D r_T^2 N_o) \quad (5257)$$

$$\tau^{11}_{\gamma,\delta,w} = \sum_{\epsilon \in A} Z^*_{\delta,\epsilon} \tau^1_{\gamma,\epsilon,w} \tau^{10}_{\gamma,\epsilon,w} \quad (3r_D r_T^3) \quad (5258)$$

$$\tau^{12}_{\gamma,\delta,w} = \sum_{\epsilon \in A} Z_{\gamma,\epsilon} \tau^{11}_{\epsilon,\delta,w} \quad (2r_D r_T^3) \quad (5259)$$

$${}^2R^2_{i,\gamma} \leftarrow \sum_{\delta \in A} \sum_{w \in D} \frac{1}{4} {}^2D^2_{i,w} Y^2_{i,\delta} \tau^0_{\delta,\gamma,w} \tau^{12}_{\delta,\gamma,w} \quad (4r_D r_T^2 N_o) \quad \tau^{11}_{\gamma,\delta,w} = \sum_{\epsilon \in A} Z^*_{\delta,\epsilon} \tau^{10}_{\gamma,\epsilon,w} \tau^9_{\gamma,\epsilon,w} \quad (3r_D r_T^3) \quad (5273)$$

$$(5260)$$

Raw expression

$$\tau^{12}_{\gamma,\delta,w} = \sum_{\epsilon \in A} Z_{\gamma,\epsilon} \tau^{11}_{\epsilon,\delta,w} \quad (2r_D r_T^3) \quad (5274)$$

$${}^2R^2_{i,\epsilon} \leftarrow \sum_{\gamma \in A} \sum_{j \in O} \sum_{k \in O} \sum_{l \in O} \sum_{a \in V} \sum_{b \in V} \sum_{c \in V} \sum_{d \in V} \frac{1}{4} Y^{1,*}_{a,\epsilon} Z^*_{\epsilon,\gamma} Y^{3,*}_{b,\gamma} Y^{4,*}_{j,\gamma} {}^2D^{a,i,b,j} {}^2T_{a,i,c,k} {}^2T_{d,j,b,l} V_{k,d,l,c} \quad (5261)$$

$${}^2R^2_{i,\gamma} \leftarrow \sum_{\delta \in A} \sum_{w \in D} \frac{1}{4} {}^2D^2_{i,w} \tau^7_{\delta,i} \tau^{12}_{\delta,\gamma,w} \tau^8_{\delta,\gamma,w} \quad (4r_D r_T^2 N_o) \quad (5275)$$

Factorized expression

Raw expression

$$\tau^0_{\gamma,\alpha} = \sum_{a \in V} W^2_{a,\alpha} Y^1_{a,\gamma} \quad (2r_T r_V N_v) \quad (5262)$$

$${}^2R^2_{i,\epsilon} \leftarrow \sum_{\gamma \in A} \sum_{j \in O} \sum_{k \in O} \sum_{l \in O} \sum_{a \in V} \sum_{b \in V} \sum_{c \in V} \sum_{d \in V} \frac{1}{4} Y^{1,*}_{a,\epsilon} Z^*_{\epsilon,\gamma} Y^{3,*}_{b,\gamma} Y^{4,*}_{j,\gamma} {}^2D^{a,i,b,j} {}^2T_{a,k,b,l} {}^2T_{c,i,d,j} V_{k,c,l,d} \quad (5276)$$

$$\tau^1_{\gamma,\alpha,i} = \sum_{\beta \in B} W^1_{i,\beta} X_{\beta,\alpha} \tau^0_{\gamma,\beta} \quad (3r_T r_V^2 N_o) \quad (5263)$$

Factorized expression

$$\tau^2_{\gamma,\alpha} = \sum_{i \in O} W^3_{i,\alpha} Y^2_{i,\gamma} \quad (2r_T r_V N_o) \quad (5264)$$

$$\tau^0_{\gamma,\delta,w} = \sum_{a \in V} {}^2D^1_{a,w} Y^1_{a,\gamma} Y^{1,*}_{a,\delta} \quad (3r_D r_T^2 N_v) \quad (5277)$$

$$\tau^3_{\gamma,\alpha} = \sum_{a \in V} W^4_{a,\alpha} Y^3_{a,\gamma} \quad (2r_T r_V N_v) \quad (5265)$$

$$\tau^1_{\gamma,\alpha} = \sum_{a \in V} W^2_{a,\alpha} Y^1_{a,\gamma} \quad (2r_T r_V N_v) \quad (5278)$$

$$\tau^4_{\gamma,\delta,i} = \sum_{\alpha \in B} \tau^2_{\gamma,\alpha} \tau^3_{\delta,\alpha} \tau^1_{\gamma,\alpha,i} \quad (3r_T^2 r_V N_o) \quad (5266)$$

$$\tau^2_{\gamma,\alpha,i} = \sum_{\beta \in B} W^1_{i,\beta} X_{\beta,\alpha} \tau^1_{\gamma,\beta} \quad (3r_T r_V^2 N_o) \quad (5279)$$

$$\tau^5_{\gamma,i} = \sum_{\delta \in A} Z_{\delta,\gamma} \tau^4_{\delta,\gamma,i} \quad (2r_T^2 N_o) \quad (5267)$$

$$\tau^3_{\gamma,\alpha} = \sum_{i \in O} W^3_{i,\alpha} Y^2_{i,\gamma} \quad (2r_T r_V N_o) \quad (5280)$$

$$\tau^6_{i,j} = \sum_{\gamma \in A} Y^4_{j,\gamma} \tau^5_{\gamma,i} \quad (2r_T N_o^2) \quad (5268)$$

$$\tau^4_{\gamma,\alpha} = \sum_{a \in V} W^4_{a,\alpha} Y^3_{a,\gamma} \quad (2r_T r_V N_v) \quad (5281)$$

$$\tau^7_{\gamma,i} = \sum_{j \in O} Y^2_{j,\gamma} \tau^6_{j,i} \quad (2r_T N_o^2) \quad (5269)$$

$$\tau^5_{\gamma,\delta,i} = \sum_{\alpha \in B} \tau^3_{\gamma,\alpha} \tau^4_{\delta,\alpha} \tau^2_{\gamma,\alpha,i} \quad (3r_T^2 r_V N_o) \quad (5282)$$

$$\tau^8_{\gamma,\delta,w} = \sum_{a \in V} {}^2D^1_{a,w} Y^1_{a,\gamma} Y^{1,*}_{a,\delta} \quad (3r_D r_T^2 N_v) \quad (5270)$$

$$\tau^6_{\gamma,\delta,\epsilon} = \sum_{i \in O} Y^2_{i,\delta} Z_{\delta,\epsilon} \tau^5_{\gamma,\epsilon,i} \quad (3r_T^3 N_o) \quad (5283)$$

$$\tau^9_{\gamma,\delta,w} = \sum_{a \in V} {}^2D^3_{a,w} Y^3_{a,\gamma} Y^{3,*}_{a,\delta} \quad (3r_D r_T^2 N_v) \quad (5271)$$

$$\tau^7_{\gamma,\delta,i} = \sum_{\epsilon \in A} Y^4_{i,\epsilon} \tau^6_{\gamma,\delta,\epsilon} \quad (2r_T^3 N_o) \quad (5284)$$

$$\tau^{10}_{\gamma,\delta,w} = \sum_{i \in O} {}^2D^4_{i,w} Y^4_{i,\gamma} Y^{4,*}_{i,\delta} \quad (3r_D r_T^2 N_o) \quad (5272)$$

$$\tau^8_{\gamma,\delta,w} = \sum_{a \in V} {}^2D^3_{a,w} Y^3_{a,\gamma} Y^{3,*}_{a,\delta} \quad (3r_D r_T^2 N_v) \quad (5285)$$

$$\tau_{\gamma,\delta,w}^9 = \sum_{i \in O} {}^2D_{i,w}^4 Y_{i,\gamma}^4 Y_{i,\delta}^{4,*} \quad (3r_D r_T^2 N_o) \quad (5286)$$

$$\tau_{\gamma,\delta,i}^6 = \sum_{\alpha \in B} \tau_{\delta,\alpha}^4 \tau_{\gamma,\alpha}^5 \tau_{\delta,\alpha,i}^3 \quad (3r_T^2 r_V N_o) \quad (5299)$$

$$\tau_{\gamma,\delta,w}^{10} = \sum_{\epsilon \in A} Z_{\delta,\epsilon}^* \tau_{\gamma,\epsilon,w}^8 \tau_{\gamma,\epsilon,w}^9 \quad (3r_D r_T^3) \quad (5287)$$

$$\tau_{\gamma,i}^7 = \sum_{\delta \in A} Z_{\gamma,\delta} \tau_{\gamma,\delta,i}^6 \quad (2r_T^2 N_o) \quad (5300)$$

$$\tau_{\gamma,\delta,w}^{11} = \sum_{\epsilon \in A} Z_{\gamma,\epsilon} \tau_{\epsilon,\delta,w}^{10} \quad (2r_D r_T^3) \quad (5288)$$

$$\tau_{i,j}^8 = \sum_{\gamma \in A} Y_{j,\gamma}^2 \tau_{\gamma,i}^7 \quad (2r_T N_o^2) \quad (5301)$$

$$\tau_{\gamma,\delta,w,i}^{12} = \sum_{\epsilon \in A} \tau_{\epsilon,\delta,w}^{11} \tau_{\epsilon,\gamma,i}^7 \quad (2r_D r_T^3 N_o) \quad (5289)$$

$$\tau_{\gamma,i}^9 = \sum_{j \in O} Y_{j,\gamma}^4 \tau_{j,i}^8 \quad (2r_T N_o^2) \quad (5302)$$

$$\tau_{\gamma,w,i}^{13} = \sum_{\delta \in A} \tau_{\delta,\gamma,w}^0 \tau_{\delta,\gamma,w,i}^{12} \quad (2r_D r_T^2 N_o) \quad (5290)$$

$$\tau_{\gamma,\delta,w}^{10} = \sum_{i \in O} {}^2D_{i,w}^4 Y_{i,\delta}^{4,*} \tau_{\gamma,i}^9 \quad (3r_D r_T^2 N_o) \quad (5303)$$

$${}^2R_{i,\gamma}^2 \leftarrow \sum_{w \in D} \frac{1}{4} {}^2D_{i,w}^2 \tau_{\gamma,w,i}^{13} \quad (2r_D r_T N_o) \quad (5291)$$

$$\tau_{\gamma,\delta,w}^{11} = \sum_{\epsilon \in A} Z_{\delta,\epsilon}^* \tau_{\gamma,\epsilon,w}^1 \tau_{\gamma,\epsilon,w}^{10} \quad (3r_D r_T^3) \quad (5304)$$

Raw expression

$${}^2R_{i,\epsilon}^2 \leftarrow \sum_{\gamma \in A} \sum_{j \in O} \sum_{k \in O} \sum_{l \in O} \sum_{a \in V} \sum_{b \in V} \sum_{c \in V} \sum_{d \in V} \frac{1}{4} Y_{a,\epsilon}^{1,*} Z_{\epsilon,\gamma}^* Y_{b,\gamma}^{3,*} Y_{j,\gamma}^{4,*} {}^2D_{a,i,b,j} {}^2T_{a,k,b,l} {}^2T_{c,j,d,i} V_{k,d,l,c} \quad (5292)$$

$$\tau_{\gamma,\delta,w}^{12} = \sum_{\epsilon \in A} Z_{\gamma,\epsilon} \tau_{\epsilon,\delta,w}^{11} \quad (2r_D r_T^3) \quad (5305)$$

$${}^2R_{i,\gamma}^2 \leftarrow \sum_{\delta \in A} \sum_{w \in D} \frac{1}{4} {}^2D_{i,w}^2 Y_{i,\delta}^2 \tau_{\delta,\gamma,w}^0 \tau_{\delta,\gamma,w}^{12} \quad (4r_D r_T^2 N_o) \quad (5306)$$

Factorized expression

$$\tau_{\gamma,\delta,w}^0 = \sum_{a \in V} {}^2D_{a,w}^1 Y_{a,\gamma}^1 Y_{a,\delta}^{1,*} \quad (3r_D r_T^2 N_v) \quad (5293)$$

Raw expression

$${}^2R_{i,\epsilon}^2 \leftarrow \sum_{\gamma \in A} \sum_{j \in O} \sum_{k \in O} \sum_{l \in O} \sum_{a \in V} \sum_{b \in V} \sum_{c \in V} \sum_{d \in V} \frac{1}{4} Y_{a,\epsilon}^{1,*} Z_{\epsilon,\gamma}^* Y_{b,\gamma}^{3,*} Y_{j,\gamma}^{4,*} {}^2D_{a,i,b,j} {}^2T_{a,k,c,i} {}^2T_{b,j,d,l} V_{k,d,l,c} \quad (5307)$$

$$\tau_{\gamma,\delta,w}^1 = \sum_{a \in V} {}^2D_{a,w}^3 Y_{a,\gamma}^3 Y_{a,\delta}^{3,*} \quad (3r_D r_T^2 N_v) \quad (5294)$$

Factorized expression

$$\tau_{\gamma,\alpha}^2 = \sum_{a \in V} W_{a,\alpha}^2 Y_{a,\gamma}^3 \quad (2r_T r_V N_v) \quad (5295)$$

$$\tau_{\gamma,\delta,w}^0 = \sum_{a \in V} {}^2D_{a,w}^1 Y_{a,\gamma}^1 Y_{a,\delta}^{1,*} \quad (3r_D r_T^2 N_v) \quad (5308)$$

$$\tau_{\gamma,\alpha,i}^3 = \sum_{\beta \in B} W_{i,\beta}^1 X_{\beta,\alpha} \tau_{\gamma,\beta}^2 \quad (3r_T r_V^2 N_o) \quad (5296)$$

$$\tau_{\gamma,\alpha}^1 = \sum_{a \in V} W_{a,\alpha}^4 Y_{a,\gamma}^1 \quad (2r_T r_V N_v) \quad (5309)$$

$$\tau_{\gamma,\alpha}^4 = \sum_{i \in O} W_{i,\alpha}^3 Y_{i,\gamma}^4 \quad (2r_T r_V N_o) \quad (5297)$$

$$\tau_{\gamma,\alpha,i}^2 = \sum_{\beta \in B} X_{\alpha,\beta} W_{i,\beta}^3 \tau_{\gamma,\beta}^1 \quad (3r_T r_V^2 N_o) \quad (5310)$$

$$\tau_{\gamma,\alpha}^5 = \sum_{a \in V} W_{a,\alpha}^4 Y_{a,\gamma}^1 \quad (2r_T r_V N_v) \quad (5298)$$

$$\tau_{\gamma,\alpha}^3 = \sum_{i \in O} W_{i,\alpha}^1 Y_{i,\gamma}^2 \quad (2r_T r_V N_o) \quad (5311)$$



$$\tau^4_{\gamma,\alpha} = \sum_{\delta \in A} \sum_{i \in O} Z_{\delta,\gamma} Y^4_{i,\gamma} \tau^3_{\delta,\alpha} \tau^2_{\delta,\alpha,i} \quad (4r_T^2 r_V N_o) \quad (5312)$$

$$\tau^5_{\gamma,a} = \sum_{\alpha \in B} W^2_{a,\alpha} \tau^4_{\gamma,\alpha} \quad (2r_T r_V N_v) \quad (5313)$$

$$\tau^6_{a,b} = \sum_{\gamma \in A} Y^3_{b,\gamma} \tau^5_{\gamma,a} \quad (2r_T N_v^2) \quad (5314)$$

$$\tau^7_{\gamma,a} = \sum_{b \in V} Y^3_{b,\gamma} \tau^6_{b,a} \quad (2r_T N_v^2) \quad (5315)$$

$$\tau^8_{\gamma,\delta,w} = \sum_{a \in V} {}^2D^3_{a,w} Y^{3,*}_{a,\delta} \tau^7_{\gamma,a} \quad (3r_D r_T^2 N_v) \quad (5316)$$

$$\tau^9_{\gamma,\delta,w} = \sum_{i \in O} {}^2D^4_{i,w} Y^4_{i,\gamma} Y^{4,*}_{i,\delta} \quad (3r_D r_T^2 N_o) \quad (5317)$$

$$\tau^{10}_{\gamma,\delta,w} = \sum_{\epsilon \in A} Z^*_{\delta,\epsilon} \tau^8_{\gamma,\epsilon,w} \tau^9_{\gamma,\epsilon,w} \quad (3r_D r_T^3) \quad (5318)$$

$$\tau^{11}_{\gamma,\delta,w} = \sum_{\epsilon \in A} Z_{\gamma,\epsilon} \tau^{10}_{\epsilon,\delta,w} \quad (2r_D r_T^3) \quad (5319)$$

$${}^2R^2_{i,\gamma} \leftarrow \sum_{\delta \in A} \sum_{w \in D} \frac{1}{4} {}^2D^2_{i,w} Y^2_{i,\delta} \tau^0_{\delta,\gamma,w} \tau^{11}_{\delta,\gamma,w} \quad (4r_D r_T^2 N_o) \quad (5320)$$

Raw expression

$${}^2R^2_{i,\epsilon} \leftarrow \sum_{\gamma \in A} \sum_{j \in O} \sum_{k \in O} \sum_{l \in O} \sum_{a \in V} \sum_{b \in V} \sum_{c \in V} \sum_{d \in V} \frac{1}{4} Y^{1,*}_{a,\epsilon} Z^*_{\epsilon,\gamma} Y^{3,*}_{b,\gamma} Y^{4,*}_{j,\gamma} {}^2D^{a,i,b,j} {}^2T_{a,k,c,i} {}^2T_{b,l,d,j} V_{k,c,l,d} \quad (5321)$$

Factorized expression

$$\tau^0_{\gamma,\alpha} = \sum_{a \in V} W^4_{a,\alpha} Y^1_{a,\gamma} \quad (2r_T r_V N_v) \quad (5322)$$

$$\tau^1_{\gamma,\alpha,i} = \sum_{\beta \in B} X_{\alpha,\beta} W^3_{i,\beta} \tau^0_{\gamma,\beta} \quad (3r_T r_V^2 N_o) \quad (5323)$$

$$\tau^2_{\gamma,\alpha} = \sum_{a \in V} W^2_{a,\alpha} Y^3_{a,\gamma} \quad (2r_T r_V N_v) \quad (5324)$$

$$\tau^3_{\gamma,\alpha,i} = \sum_{\delta \in A} Z_{\gamma,\delta} Y^4_{i,\delta} \tau^2_{\delta,\alpha} \quad (3r_T^2 r_V N_o) \quad (5325)$$

$$\tau^4_{\gamma,i,j,k} = \sum_{\alpha \in B} W^1_{i,\alpha} \tau^1_{\gamma,\alpha,j} \tau^3_{\gamma,\alpha,k} \quad (3r_T r_V N_o^3) \quad (5326)$$

$$\tau^5_{i,j,k,l} = \sum_{\gamma \in A} Y^2_{k,\gamma} \tau^4_{\gamma,i,j,l} \quad (2r_T N_o^4) \quad (5327)$$

$$\tau^6_{\gamma,i,j,k} = \sum_{l \in O} Y^4_{l,\gamma} \tau^5_{i,l,j,k} \quad (2r_T N_o^4) \quad (5328)$$

$$\tau^7_{\gamma,\delta,w} = \sum_{a \in V} {}^2D^3_{a,w} Y^3_{a,\gamma} Y^{3,*}_{a,\delta} \quad (3r_D r_T^2 N_v) \quad (5329)$$

$$\tau^8_{\gamma,\delta,w,i} = \sum_{\epsilon \in A} Z^*_{\delta,\epsilon} Y^{4,*}_{i,\epsilon} \tau^7_{\gamma,\epsilon,w} \quad (3r_D r_T^3 N_o) \quad (5330)$$

$$\tau^9_{\gamma,\delta,w} = \sum_{a \in V} {}^2D^1_{a,w} Y^1_{a,\gamma} Y^{1,*}_{a,\delta} \quad (3r_D r_T^2 N_v) \quad (5331)$$

$$\tau^{10}_{\gamma,\delta,w,i} = \sum_{\epsilon \in A} Y^2_{i,\epsilon} Z_{\epsilon,\gamma} \tau^9_{\epsilon,\delta,w} \quad (3r_D r_T^3 N_o) \quad (5332)$$

$$\tau^{11}_{\gamma,w,i,j} = \sum_{\delta \in A} \sum_{k \in O} \tau^{10}_{\delta,\gamma,w,k} \tau^6_{\delta,k,i,j} \tau^8_{\delta,\gamma,w,i} \quad (3r_D r_T^2 N_o^3) \quad (5333)$$

$${}^2R^2_{i,\gamma} \leftarrow \sum_{w \in D} \sum_{j \in O} \frac{1}{4} {}^2D^2_{i,w} {}^2D^4_{j,w} \tau^{11}_{\gamma,w,j,i} \quad (3r_D r_T N_o^2) \quad (5334)$$

Raw expression

$${}^2R^2_{i,\epsilon} \leftarrow \sum_{\gamma \in A} \sum_{j \in O} \sum_{k \in O} \sum_{l \in O} \sum_{a \in V} \sum_{b \in V} \sum_{c \in V} \sum_{d \in V} \frac{1}{4} Y^{1,*}_{a,\epsilon} Z^*_{\epsilon,\gamma} Y^{3,*}_{b,\gamma} Y^{4,*}_{j,\gamma} {}^2D^{a,i,b,j} {}^2T_{a,k,c,i} {}^2T_{d,j,b,l} V_{k,c,l,d} \quad (5335)$$

Factorized expression

$$\tau^0_{\gamma,\delta,w} = \sum_{a \in V} {}^2D^1_{a,w} Y^1_{a,\gamma} Y^{1,*}_{a,\delta} \quad (3r_D r_T^2 N_v) \quad (5336)$$

$$\tau^1_{\gamma,\delta,w} = \sum_{a \in V} {}^2D^3_{a,w} Y^3_{a,\gamma} Y^{3,*}_{a,\delta} \quad (3r_D r_T^2 N_v) \quad (5337)$$

$$\tau^2_{\gamma,\alpha} = \sum_{a \in V} W^4_{a,\alpha} Y^1_{a,\gamma} \quad (2r_T r_V N_v) \quad (5338)$$

$$\tau^0_{\gamma,\delta,w} = \sum_{a \in V} {}^2D^1_{a,w} Y^1_{a,\gamma} Y^{1,*}_{a,\delta} \quad (3r_D r_T^2 N_v) \quad (5351)$$

$$\tau^3_{\gamma,\alpha,i} = \sum_{\delta \in A} Y^2_{i,\delta} Z_{\delta,\gamma} \tau^2_{\delta,\alpha} \quad (3r_T^2 r_V N_o) \quad (5339)$$

$$\tau^1_{\gamma,\delta,w} = \sum_{a \in V} {}^2D^3_{a,w} Y^1_{a,\gamma} Y^{3,*}_{a,\delta} \quad (3r_D r_T^2 N_v) \quad (5352)$$

$$\tau^4_{\gamma,\alpha} = \sum_{i \in O} W^3_{i,\alpha} Y^4_{i,\gamma} \quad (2r_T r_V N_o) \quad (5340)$$

$$\tau^2_{\gamma,\delta,w} = \sum_{i \in O} {}^2D^4_{i,w} Y^2_{i,\gamma} Y^{4,*}_{i,\delta} \quad (3r_D r_T^2 N_o) \quad (5353)$$

$$\tau^5_{\gamma,\alpha,w} = \sum_{\delta \in A} \sum_{i \in O} {}^2D^4_{i,w} Y^{4,*}_{i,\gamma} \tau^4_{\delta,\alpha} \tau^1_{\delta,\gamma,w} \tau^3_{\delta,\alpha,i} \quad (5r_D r_T^2 r_V N_o) \quad (5341)$$

$$\tau^4_{\gamma,\delta,w} = \sum_{\epsilon \in A} Z_{\epsilon,\gamma} \tau^3_{\epsilon,\delta,w} \quad (2r_D r_T^3) \quad (5355)$$

$$\tau^6_{\gamma,\alpha,w} = \sum_{\beta \in B} X_{\alpha,\beta} \tau^5_{\gamma,\beta,w} \quad (2r_D r_T r_V^2) \quad (5342)$$

$$\tau^5_{\gamma,\alpha} = \sum_{a \in V} W^2_{a,\alpha} Y^3_{a,\gamma} \quad (2r_T r_V N_v) \quad (5356)$$

$$\tau^7_{\gamma,\alpha,w} = \sum_{\delta \in A} Z^*_{\gamma,\delta} \tau^6_{\delta,\alpha,w} \quad (2r_D r_T^2 r_V) \quad (5343)$$

$$\tau^6_{\gamma,\alpha,i} = \sum_{\beta \in B} W^1_{i,\beta} X_{\beta,\alpha} \tau^5_{\gamma,\beta} \quad (3r_T r_V^2 N_o) \quad (5357)$$

$$\tau^8_{\gamma,\alpha} = \sum_{i \in O} W^1_{i,\alpha} Y^2_{i,\gamma} \quad (2r_T r_V N_o) \quad (5344)$$

$$\tau^7_{\gamma,\alpha} = \sum_{i \in O} W^3_{i,\alpha} Y^4_{i,\gamma} \quad (2r_T r_V N_o) \quad (5358)$$

$$\tau^9_{\gamma,\alpha} = \sum_{a \in V} W^2_{a,\alpha} Y^3_{a,\gamma} \quad (2r_T r_V N_v) \quad (5345)$$

$$\tau^8_{\gamma,\alpha} = \sum_{a \in V} W^4_{a,\alpha} Y^3_{a,\gamma} \quad (2r_T r_V N_v) \quad (5359)$$

$$\tau^{10}_{\gamma,\alpha,i} = \sum_{\delta \in A} Z_{\gamma,\delta} Y^4_{i,\delta} \tau^9_{\delta,\alpha} \quad (3r_T^2 r_V N_o) \quad (5346)$$

$$\tau^9_{\gamma,\delta,i} = \sum_{\alpha \in B} \tau^7_{\gamma,\alpha} \tau^8_{\delta,\alpha} \tau^6_{\gamma,\alpha,i} \quad (3r_T^2 r_V N_o) \quad (5360)$$

$$\tau^{11}_{\gamma,\delta,w,i} = \sum_{\alpha \in B} \tau^8_{\gamma,\alpha} \tau^{10}_{\gamma,\alpha,i} \tau^7_{\delta,\alpha,w} \quad (3r_D r_T^2 r_V N_o) \quad (5347)$$

$$\tau^{10}_{\gamma,\delta,\epsilon} = \sum_{i \in O} Y^2_{i,\gamma} Z_{\gamma,\delta} \tau^9_{\epsilon,\delta,i} \quad (3r_T^3 N_o) \quad (5361)$$

$$\tau^{12}_{\gamma,w,i} = \sum_{\delta \in A} \tau^0_{\delta,\gamma,w} \tau^{11}_{\delta,\gamma,w,i} \quad (2r_D r_T^2 N_o) \quad (5348)$$

$$\tau^{11}_{\gamma,\delta,i} = \sum_{\epsilon \in A} Y^4_{i,\epsilon} \tau^{10}_{\gamma,\epsilon,\delta} \quad (2r_T^3 N_o) \quad (5362)$$

$${}^2R^2_{i,\gamma} \leftarrow \sum_{w \in D} \frac{1}{4} {}^2D^2_{i,w} \tau^{12}_{\gamma,w,i} \quad (2r_D r_T N_o) \quad (5349)$$

$$\tau^{12}_{\gamma,\delta,w,i} = \sum_{\epsilon \in A} \tau^{11}_{\gamma,\epsilon,i} \tau^4_{\epsilon,\delta,w} \quad (2r_D r_T^3 N_o) \quad (5363)$$

Raw expression

$${}^2R^2_{i,\epsilon} \leftarrow \sum_{\gamma \in A} \sum_{j \in O} \sum_{k \in O} \sum_{l \in O} \sum_{a \in V} \sum_{b \in V} \sum_{c \in V} \sum_{d \in V} \frac{1}{4} Y^{1,*}_{a,\epsilon} Z^*_{\epsilon,\gamma} Y^{3,*}_{b,\gamma} Y^{4,*}_{j,\gamma} {}^2D^{a,i,b,j} {}^2T_{a,k,c,i} {}^2T_{d,l,b,j} V_{k,d,l,c} \quad (5350)$$

$$\tau^{13}_{\gamma,w,i} = \sum_{\delta \in A} \tau^0_{\delta,\gamma,w} \tau^{12}_{\delta,\gamma,w,i} \quad (2r_D r_T^2 N_o) \quad (5364)$$

Factorized expression

$${}^2R^2_{i,\gamma} \leftarrow \sum_{w \in D} \frac{1}{4} {}^2D^2_{i,w} \tau^{13}_{\gamma,w,i} \quad (2r_D r_T N_o) \quad (5365)$$

Raw expression

$${}^2R^2_{i,\epsilon} \leftarrow \sum_{\gamma \in A} \sum_{j \in O} \sum_{k \in O} \sum_{l \in O} \sum_{a \in V} \sum_{b \in V} \sum_{c \in V} \sum_{d \in V} \frac{1}{4} Y^{1,*}_{a,\epsilon} Z^*_{\epsilon,\gamma} Y^{3,*}_{b,\gamma} Y^{4,*}_{j,\gamma} {}^2D^{a,i,b,j} {}^2T_{a,k,d,l} {}^2T_{b,j,c,i} V_{k,d,l,c} \quad (5366)$$

Factorized expression

$$\tau^0_{\gamma,\delta,w} = \sum_{a \in V} {}^2D^3_{a,w} Y^1_{a,\gamma} Y^{3,*}_{a,\delta} \quad (3r_D r_T^2 N_v) \quad (5367)$$

$$\tau^1_{\gamma,\delta,w} = \sum_{i \in O} {}^2D^4_{i,w} Y^2_{i,\gamma} Y^{4,*}_{i,\delta} \quad (3r_D r_T^2 N_o) \quad (5368)$$

$$\tau^2_{\gamma,\delta,w} = \sum_{\epsilon \in A} Z^*_{\delta,\epsilon} \tau^0_{\gamma,\epsilon,w} \tau^1_{\gamma,\epsilon,w} \quad (3r_D r_T^3) \quad (5369)$$

$$\tau^3_{\gamma,\delta,w} = \sum_{\epsilon \in A} Z_{\epsilon,\gamma} \tau^2_{\epsilon,\delta,w} \quad (2r_D r_T^3) \quad (5370)$$

$$\tau^4_{\gamma,\alpha} = \sum_{a \in V} W^2_{a,\alpha} Y^3_{a,\gamma} \quad (2r_T r_V N_v) \quad (5371)$$

$$\tau^5_{\gamma,\alpha,i} = \sum_{\beta \in B} W^1_{i,\beta} X_{\beta,\alpha} \tau^4_{\gamma,\beta} \quad (3r_T r_V^2 N_o) \quad (5372)$$

$$\tau^6_{\gamma,\alpha} = \sum_{i \in O} W^3_{i,\alpha} Y^4_{i,\gamma} \quad (2r_T r_V N_o) \quad (5373)$$

$$\tau^7_{\gamma,\alpha} = \sum_{\delta \in A} \sum_{i \in O} Y^2_{i,\gamma} Z_{\gamma,\delta} \tau^6_{\delta,\alpha} \tau^5_{\delta,\alpha,i} \quad (4r_T^2 r_V N_o) \quad (5374)$$

$$\tau^8_{\gamma,a} = \sum_{\alpha \in B} W^4_{a,\alpha} \tau^7_{\gamma,\alpha} \quad (2r_T r_V N_v) \quad (5375)$$

$$\tau^9_{\gamma,\delta} = \sum_{a \in V} Y^3_{a,\delta} \tau^8_{\gamma,a} \quad (2r_T^2 N_v) \quad (5376)$$

$$\tau^{10}_{\gamma,a} = \sum_{\delta \in A} Y^1_{a,\delta} \tau^9_{\delta,\gamma} \quad (2r_T^2 N_v) \quad (5377)$$

$$\tau^{11}_{\gamma,\delta,w} = \sum_{a \in V} {}^2D^1_{a,w} Y^{1,*}_{a,\delta} \tau^{10}_{\gamma,a} \quad (3r_D r_T^2 N_v) \quad (5378)$$

$${}^2R^2_{i,\gamma} \leftarrow \sum_{\delta \in A} \sum_{w \in D} \frac{1}{4} {}^2D^2_{i,w} Y^4_{i,\delta} \tau^{11}_{\delta,\gamma,w} \tau^3_{\delta,\gamma,w} \quad (4r_D r_T^2 N_o) \quad (5379)$$

Raw expression

$${}^2R^2_{i,\epsilon} \leftarrow \sum_{\gamma \in A} \sum_{j \in O} \sum_{k \in O} \sum_{l \in O} \sum_{a \in V} \sum_{b \in V} \sum_{c \in V} \sum_{d \in V} \frac{1}{4} Y^{1,*}_{a,\epsilon} Z^*_{\epsilon,\gamma} Y^{3,*}_{b,\gamma} Y^{4,*}_{j,\gamma} {}^2D^{a,i,b,j} {}^2T_{a,k,d,l} {}^2T_{c,i,b,j} V_{k,d,l,c} \quad (5380)$$

Factorized expression

$$\tau^0_{\gamma,\delta,w} = \sum_{a \in V} {}^2D^3_{a,w} Y^1_{a,\gamma} Y^{3,*}_{a,\delta} \quad (3r_D r_T^2 N_v) \quad (5381)$$

$$\tau^1_{\gamma,\delta,w,i} = \sum_{\epsilon \in A} Z^*_{\delta,\epsilon} Y^{4,*}_{i,\epsilon} \tau^0_{\gamma,\epsilon,w} \quad (3r_D r_T^3 N_o) \quad (5382)$$

$$\tau^2_{\gamma,\delta,\epsilon,w} = \sum_{i \in O} {}^2D^4_{i,w} Y^4_{i,\delta} \tau^1_{\gamma,\epsilon,w,i} \quad (3r_D r_T^3 N_o) \quad (5383)$$

$$\tau^3_{\gamma,\delta,w} = \sum_{a \in V} {}^2D^1_{a,w} Y^1_{a,\gamma} Y^{1,*}_{a,\delta} \quad (3r_D r_T^2 N_v) \quad (5384)$$

$$\tau^4_{\gamma,\delta,w,i} = \sum_{\epsilon \in A} Y^2_{i,\epsilon} Z_{\epsilon,\gamma} \tau^3_{\epsilon,\delta,w} \quad (3r_D r_T^3 N_o) \quad (5385)$$

$$\tau^5_{\gamma,\delta,\alpha,w} = \sum_{i \in O} W^1_{i,\alpha} \tau^4_{\gamma,\delta,w,i} \quad (2r_D r_T^2 r_V N_o) \quad (5386)$$

$$\tau^6_{\gamma,\alpha} = \sum_{a \in V} W^4_{a,\alpha} Y^3_{a,\gamma} \quad (2r_T r_V N_v) \quad (5387)$$

$$\tau^7_{\gamma,\alpha,i} = \sum_{\beta \in B} X_{\alpha,\beta} W^3_{i,\beta} \tau^6_{\gamma,\beta} \quad (3r_T r_V^2 N_o) \quad (5388)$$

$$\tau^8_{\gamma,\delta,\alpha} = \sum_{i \in O} Y^2_{i,\gamma} \tau^7_{\delta,\alpha,i} \quad (2r_T^2 r_V N_o) \quad (5389)$$

$$\tau^9_{\gamma,\delta,\alpha,w} = \sum_{\epsilon \in A} \tau^8_{\gamma,\epsilon,\alpha} \tau^2_{\gamma,\epsilon,\delta,w} \tau^5_{\epsilon,\delta,\alpha,w} \quad (3r_D r_T^3 r_V) \quad (5390)$$

$$\tau^{10}_{\gamma,\alpha} = \sum_{a \in V} W^2_{a,\alpha} Y^3_{a,\gamma} \quad (2r_T r_V N_v) \quad (5391)$$

$$\tau^{11}_{\gamma,\alpha,i} = \sum_{\delta \in A} Z_{\gamma,\delta} Y^4_{i,\delta} \tau^{10}_{\delta,\alpha} \quad (3r_T^2 r_V N_o) \quad (5392)$$

$$\tau^9_{\gamma,\delta,w} = \sum_{a \in V} {}^2D^1_{a,w} Y^1_{a,\gamma} Y^{1,*}_{a,\delta} \quad (3r_D r_T^2 N_v) \quad (5405)$$

$$\tau^{12}_{\gamma,w,i} = \sum_{\delta \in A} \sum_{\alpha \in B} \tau^{11}_{\delta,\alpha,i} \tau^9_{\delta,\gamma,\alpha,w} \quad (2r_D r_T^2 r_V N_o) \quad (5393)$$

$$\tau^{10}_{\gamma,\delta,w,i} = \sum_{\epsilon \in A} Y^2_{i,\epsilon} Z_{\epsilon,\gamma} \tau^9_{\epsilon,\delta,w} \quad (3r_D r_T^3 N_o) \quad (5406)$$

$${}^2R^2_{i,\gamma} \leftarrow \sum_{w \in D} \frac{1}{4} {}^2D^2_{i,w} \tau^{12}_{\gamma,w,i} \quad (2r_D r_T N_o) \quad (5394)$$

$$\tau^{11}_{\gamma,w,i,j} = \sum_{\delta \in A} \sum_{k \in O} \tau^{10}_{\delta,\gamma,w,k} \tau^6_{\delta,k,i,j} \tau^8_{\delta,\gamma,w,j} \quad (3r_D r_T^2 N_o^3) \quad (5407)$$

Raw expression

$${}^2R^2_{i,\epsilon} \leftarrow \sum_{\gamma \in A} \sum_{j \in O} \sum_{k \in O} \sum_{l \in O} \sum_{a \in V} \sum_{b \in V} \sum_{c \in V} \sum_{d \in V} \frac{1}{4} Y^{1,*}_{a,\epsilon} Z^*_{\epsilon,\gamma} Y^{3,*}_{b,\gamma} Y^{4,*}_{j,\gamma} {}^2D^{a,i,b,j} {}^2T_{a,l,b,j} {}^2T_{c,i,d,k} V_{l,d,k,c} \quad (5395)$$

$${}^2R^2_{i,\gamma} \leftarrow \sum_{w \in D} \sum_{j \in O} \frac{1}{4} {}^2D^2_{i,w} {}^2D^4_{j,w} \tau^{11}_{\gamma,w,i,j} \quad (3r_D r_T N_o^2) \quad (5408)$$

Raw expression

$${}^2R^2_{i,\epsilon} \leftarrow \sum_{\gamma \in A} \sum_{j \in O} \sum_{k \in O} \sum_{l \in O} \sum_{a \in V} \sum_{b \in V} \sum_{c \in V} \sum_{d \in V} \frac{1}{4} Y^{1,*}_{a,\epsilon} Z^*_{\epsilon,\gamma} Y^{3,*}_{b,\gamma} Y^{4,*}_{j,\gamma} {}^2D^{a,i,b,j} {}^2T_{a,l,b,j} {}^2T_{c,k,d,i} V_{l,c,k,d} \quad (5409)$$

Factorized expression

$$\tau^0_{\gamma,\alpha} = \sum_{a \in V} W^2_{a,\alpha} Y^1_{a,\gamma} \quad (2r_T r_V N_v) \quad (5396)$$

Factorized expression

$$\tau^0_{\gamma,\alpha} = \sum_{a \in V} W^2_{a,\alpha} Y^1_{a,\gamma} \quad (2r_T r_V N_v) \quad (5410)$$

$$\tau^1_{\gamma,\alpha,i} = \sum_{\beta \in B} W^1_{i,\beta} X_{\beta,\alpha} \tau^0_{\gamma,\beta} \quad (3r_T r_V^2 N_o) \quad (5397)$$

$$\tau^1_{\gamma,\alpha,i} = \sum_{\delta \in A} Y^2_{i,\delta} Z_{\delta,\gamma} \tau^0_{\delta,\alpha} \quad (3r_T^2 r_V N_o) \quad (5411)$$

$$\tau^2_{\gamma,\alpha} = \sum_{a \in V} W^4_{a,\alpha} Y^3_{a,\gamma} \quad (2r_T r_V N_v) \quad (5398)$$

$$\tau^2_{\gamma,\alpha} = \sum_{a \in V} W^4_{a,\alpha} Y^3_{a,\gamma} \quad (2r_T r_V N_v) \quad (5412)$$

$$\tau^3_{\gamma,\alpha,i} = \sum_{\delta \in A} Z_{\gamma,\delta} Y^4_{i,\delta} \tau^2_{\delta,\alpha} \quad (3r_T^2 r_V N_o) \quad (5399)$$

$$\tau^3_{\gamma,\alpha,i} = \sum_{\beta \in B} X_{\alpha,\beta} W^3_{i,\beta} \tau^2_{\gamma,\beta} \quad (3r_T r_V^2 N_o) \quad (5413)$$

$$\tau^4_{\gamma,i,j,k} = \sum_{\alpha \in B} W^3_{j,\alpha} \tau^1_{\gamma,\alpha,i} \tau^3_{\gamma,\alpha,k} \quad (3r_T r_V N_o^3) \quad (5400)$$

$$\tau^5_{i,j,k,l} = \sum_{\gamma \in A} Y^2_{k,\gamma} \tau^4_{\gamma,i,j,l} \quad (2r_T N_o^4) \quad (5401)$$

$$\tau^4_{\gamma,\delta,\alpha} = \sum_{i \in O} Y^4_{i,\delta} \tau^3_{\gamma,\alpha,i} \quad (2r_T^2 r_V N_o) \quad (5414)$$

$$\tau^6_{\gamma,i,j,k} = \sum_{l \in O} Y^4_{l,\gamma} \tau^5_{i,l,j,k} \quad (2r_T N_o^4) \quad (5402)$$

$$\tau^5_{\gamma,\delta,w} = \sum_{a \in V} {}^2D^1_{a,w} Y^1_{a,\gamma} Y^{1,*}_{a,\delta} \quad (3r_D r_T^2 N_v) \quad (5415)$$

$$\tau^7_{\gamma,\delta,w} = \sum_{a \in V} {}^2D^3_{a,w} Y^3_{a,\gamma} Y^{3,*}_{a,\delta} \quad (3r_D r_T^2 N_v) \quad (5403)$$

$$\tau^6_{\gamma,\delta,w,i} = \sum_{\epsilon \in A} Y^2_{i,\epsilon} Z_{\epsilon,\gamma} \tau^5_{\epsilon,\delta,w} \quad (3r_D r_T^3 N_o) \quad (5416)$$

$$\tau^8_{\gamma,\delta,w,i} = \sum_{\epsilon \in A} Z^*_{\delta,\epsilon} Y^{4,*}_{i,\epsilon} \tau^7_{\gamma,\epsilon,w} \quad (3r_D r_T^3 N_o) \quad (5404)$$

$$\tau^7_{\gamma,\delta,\alpha,w} = \sum_{i \in O} W^1_{i,\alpha} \tau^6_{\gamma,\delta,w,i} \quad (2r_D r_T^2 r_V N_o) \quad (5417)$$

$$\tau_{\gamma,\delta,w}^8 = \sum_{a \in V} {}^2D_{a,w}^3 Y_{a,\gamma}^3 Y_{a,\delta}^{3,*} \quad (3r_D r_T^2 N_v) \quad (5418)$$

$$\tau_{\gamma,\delta,w,i}^9 = \sum_{\epsilon \in A} Z_{\delta,\epsilon}^* Y_{i,\epsilon}^{4,*} \tau_{\gamma,\epsilon,w}^8 \quad (3r_D r_T^3 N_o) \quad (5419)$$

$$\tau_{\gamma,\delta,\epsilon,w}^{10} = \sum_{i \in O} {}^2D_{i,w}^4 Y_{i,\delta}^4 \tau_{\gamma,\epsilon,w,i}^9 \quad (3r_D r_T^3 N_o) \quad (5420)$$

$$\tau_{\gamma,\delta,\alpha,w}^{11} = \sum_{\epsilon \in A} \tau_{\epsilon,\gamma,\alpha}^4 \tau_{\gamma,\epsilon,\delta,w}^{10} \tau_{\epsilon,\delta,\alpha,w}^7 \quad (3r_D r_T^3 r_V) \quad (5421)$$

$$\tau_{\gamma,w,i}^{12} = \sum_{\delta \in A} \sum_{\alpha \in B} \tau_{\delta,\alpha,i}^1 \tau_{\delta,\gamma,\alpha,w}^{11} \quad (2r_D r_T^2 r_V N_o) \quad (5422)$$

$${}^2R_{i,\gamma}^2 \leftarrow \sum_{w \in D} \frac{1}{4} {}^2D_{i,w}^2 \tau_{\gamma,w,i}^{12} \quad (2r_D r_T N_o) \quad (5423)$$

Raw expression

$${}^2R_{i,\epsilon}^2 \leftarrow \sum_{\gamma \in A} \sum_{j \in O} \sum_{k \in O} \sum_{l \in O} \sum_{a \in V} \sum_{b \in V} \sum_{c \in V} \sum_{d \in V} \frac{1}{4} Y_{a,\epsilon}^{1,*} Z_{\epsilon,\gamma}^* Y_{b,\gamma}^{3,*} Y_{j,\gamma}^{4,*} {}^2D_{a,i,b,j} {}^2T_{a,l,d,j} {}^2T_{b,k,c,i} V_{l,c,k,d} \quad (5424)$$

Factorized expression

$$\tau_{\gamma,\alpha}^0 = \sum_{a \in V} W_{a,\alpha}^2 Y_{a,\gamma}^3 \quad (2r_T r_V N_v) \quad (5425)$$

$$\tau_{\gamma,\alpha,i}^1 = \sum_{\beta \in B} W_{i,\beta}^1 X_{\beta,\alpha} \tau_{\gamma,\beta}^0 \quad (3r_T r_V^2 N_o) \quad (5426)$$

$$\tau_{\gamma,\alpha}^2 = \sum_{i \in O} W_{i,\alpha}^3 Y_{i,\gamma}^4 \quad (2r_T r_V N_o) \quad (5427)$$

$$\tau_{\gamma,\alpha}^3 = \sum_{a \in V} W_{a,\alpha}^4 Y_{a,\gamma}^1 \quad (2r_T r_V N_v) \quad (5428)$$

$$\tau_{\gamma,\delta,i}^4 = \sum_{\alpha \in B} \tau_{\delta,\alpha}^2 \tau_{\gamma,\alpha}^3 \tau_{\delta,\alpha,i}^1 \quad (3r_T^2 r_V N_o) \quad (5429)$$

$$\tau_{\gamma,i}^5 = \sum_{\delta \in A} Z_{\gamma,\delta} \tau_{\gamma,\delta,i}^4 \quad (2r_T^2 N_o) \quad (5430)$$

$$\tau_{i,j}^6 = \sum_{\gamma \in A} Y_{j,\gamma}^2 \tau_{\gamma,i}^5 \quad (2r_T N_o^2) \quad (5431)$$

$$\tau_{\gamma,i}^7 = \sum_{j \in O} Y_{j,\gamma}^2 \tau_{j,i}^6 \quad (2r_T N_o^2) \quad (5432)$$

$$\tau_{\gamma,\delta,w}^8 = \sum_{a \in V} {}^2D_{a,w}^1 Y_{a,\gamma}^1 Y_{a,\delta}^{1,*} \quad (3r_D r_T^2 N_v) \quad (5433)$$

$$\tau_{\gamma,\delta,w}^9 = \sum_{a \in V} {}^2D_{a,w}^3 Y_{a,\gamma}^3 Y_{a,\delta}^{3,*} \quad (3r_D r_T^2 N_v) \quad (5434)$$

$$\tau_{\gamma,\delta,w}^{10} = \sum_{i \in O} {}^2D_{i,w}^4 Y_{i,\gamma}^4 Y_{i,\delta}^{4,*} \quad (3r_D r_T^2 N_o) \quad (5435)$$

$$\tau_{\gamma,\delta,w}^{11} = \sum_{\epsilon \in A} Z_{\delta,\epsilon}^* \tau_{\gamma,\epsilon,w}^{10} \tau_{\gamma,\epsilon,w}^9 \quad (3r_D r_T^3) \quad (5436)$$

$$\tau_{\gamma,\delta,w}^{12} = \sum_{\epsilon \in A} Z_{\gamma,\epsilon} \tau_{\epsilon,\delta,w}^{11} \quad (2r_D r_T^3) \quad (5437)$$

Raw expression

$${}^2R_{i,\gamma}^2 \leftarrow \sum_{\delta \in A} \sum_{w \in D} \frac{1}{4} {}^2D_{i,w}^2 \tau_{\delta,i}^7 \tau_{\delta,\gamma,w}^{12} \tau_{\delta,\gamma,w}^8 \quad (4r_D r_T^2 N_o) \quad (5438)$$

$${}^2R_{i,\epsilon}^2 \leftarrow \sum_{\gamma \in A} \sum_{j \in O} \sum_{k \in O} \sum_{l \in O} \sum_{a \in V} \sum_{b \in V} \sum_{c \in V} \sum_{d \in V} \frac{1}{4} Y_{a,\epsilon}^{1,*} Z_{\epsilon,\gamma}^* Y_{b,\gamma}^{3,*} Y_{j,\gamma}^{4,*} {}^2D_{a,i,b,j} {}^2T_{a,l,d,j} {}^2T_{c,i,b,k} V_{l,c,k,d} \quad (5439)$$

Factorized expression

$$\tau_{\gamma,\alpha}^0 = \sum_{a \in V} W_{a,\alpha}^2 Y_{a,\gamma}^3 \quad (2r_T r_V N_v) \quad (5440)$$

$$\tau_{\gamma,\alpha,i}^1 = \sum_{\beta \in B} W_{i,\beta}^1 X_{\beta,\alpha} \tau_{\gamma,\beta}^0 \quad (3r_T r_V^2 N_o) \quad (5441)$$

$$\tau_{\gamma,\alpha}^2 = \sum_{i \in O} W_{i,\alpha}^3 Y_{i,\gamma}^4 \quad (2r_T r_V N_o) \quad (5442)$$

$$\tau_{\gamma,\alpha}^3 = \sum_{\delta \in A} \sum_{i \in O} Y_{i,\gamma}^2 Z_{\gamma,\delta} \tau_{\delta,\alpha}^2 \tau_{\delta,\alpha,i}^1 \quad (4r_T^2 r_V N_o) \quad (5443)$$

$$\tau^4_{\gamma,a} = \sum_{\alpha \in B} W^4_{a,\alpha} \tau^3_{\gamma,\alpha} \quad (2r_T r_V N_v) \quad (5444)$$

$$\tau^3_{\gamma,\alpha} = \sum_{a \in V} W^4_{a,\alpha} Y^3_{a,\gamma} \quad (2r_T r_V N_v) \quad (5457)$$

$$\tau^5_{\gamma,\delta} = \sum_{a \in V} Y^1_{a,\gamma} \tau^4_{\delta,a} \quad (2r_T^2 N_v) \quad (5445)$$

$$\tau^4_{\gamma,\delta,i} = \sum_{\alpha \in B} \tau^2_{\gamma,\alpha} \tau^3_{\delta,\alpha} \tau^1_{\gamma,\alpha,i} \quad (3r_T^2 r_V N_o) \quad (5458)$$

$$\tau^6_{\gamma,a} = \sum_{\delta \in A} Y^1_{a,\delta} \tau^5_{\gamma,\delta} \quad (2r_T^2 N_v) \quad (5446)$$

$$\tau^5_{\gamma,i} = \sum_{\delta \in A} Z_{\delta,\gamma} \tau^4_{\delta,\gamma,i} \quad (2r_T^2 N_o) \quad (5459)$$

$$\tau^7_{\gamma,\delta,w} = \sum_{a \in V} {}^2D^1_{a,w} Y^{1,*}_{a,\delta} \tau^6_{\gamma,a} \quad (3r_D r_T^2 N_v) \quad (5447)$$

$$\tau^6_{i,j} = \sum_{\gamma \in A} Y^4_{j,\gamma} \tau^5_{\gamma,i} \quad (2r_T N_o^2) \quad (5460)$$

$$\tau^8_{\gamma,\delta,w} = \sum_{a \in V} {}^2D^3_{a,w} Y^3_{a,\gamma} Y^{3,*}_{a,\delta} \quad (3r_D r_T^2 N_v) \quad (5448)$$

$$\tau^7_{\gamma,i} = \sum_{j \in O} Y^4_{j,\gamma} \tau^6_{j,i} \quad (2r_T N_o^2) \quad (5461)$$

$$\tau^9_{\gamma,\delta,w} = \sum_{i \in O} {}^2D^4_{i,w} Y^4_{i,\gamma} Y^{4,*}_{i,\delta} \quad (3r_D r_T^2 N_o) \quad (5449)$$

$$\tau^8_{\gamma,\delta,w} = \sum_{a \in V} {}^2D^3_{a,w} Y^1_{a,\gamma} Y^{3,*}_{a,\delta} \quad (3r_D r_T^2 N_v) \quad (5462)$$

$$\tau^{10}_{\gamma,\delta,w} = \sum_{\epsilon \in A} Z^*_{\delta,\epsilon} \tau^8_{\gamma,\epsilon,w} \tau^9_{\gamma,\epsilon,w} \quad (3r_D r_T^3) \quad (5450)$$

$$\tau^9_{\gamma,\delta,w} = \sum_{i \in O} {}^2D^4_{i,w} Y^2_{i,\gamma} Y^{4,*}_{i,\delta} \quad (3r_D r_T^2 N_o) \quad (5463)$$

$$\tau^{11}_{\gamma,\delta,w} = \sum_{\epsilon \in A} Z_{\gamma,\epsilon} \tau^{10}_{\epsilon,\delta,w} \quad (2r_D r_T^3) \quad (5451)$$

$$\tau^{10}_{\gamma,\delta,w} = \sum_{\epsilon \in A} Z^*_{\delta,\epsilon} \tau^8_{\gamma,\epsilon,w} \tau^9_{\gamma,\epsilon,w} \quad (3r_D r_T^3) \quad (5464)$$

$${}^2R^2_{i,\gamma} \leftarrow \sum_{\delta \in A} \sum_{w \in D} \frac{1}{4} {}^2D^2_{i,w} Y^2_{i,\delta} \tau^{11}_{\delta,\gamma,w} \tau^7_{\delta,\gamma,w} \quad (4r_D r_T^2 N_o) \quad (5452)$$

$$\tau^{11}_{\gamma,\delta,w} = \sum_{\epsilon \in A} Z_{\epsilon,\gamma} \tau^{10}_{\epsilon,\delta,w} \quad (2r_D r_T^3) \quad (5465)$$

Raw expression

$${}^2R^2_{i,\epsilon} \leftarrow \sum_{\gamma \in A} \sum_{j \in O} \sum_{k \in O} \sum_{l \in O} \sum_{a \in V} \sum_{b \in V} \sum_{c \in V} \sum_{d \in V} \frac{1}{4} Y^{1,*}_{a,\epsilon} Z^*_{\epsilon,\gamma} Y^{3,*}_{b,\gamma} Y^{4,*}_{j,\gamma} {}^2D^{a,i,b,j} {}^2T_{b,j,a,l} {}^2T_{c,i,d,k} V_{l,d,k,c} \quad (5453)$$

$$\tau^{12}_{\gamma,\delta,w} = \sum_{a \in V} {}^2D^1_{a,w} Y^3_{a,\gamma} Y^{1,*}_{a,\delta} \quad (3r_D r_T^2 N_v) \quad (5466)$$

$${}^2R^2_{i,\gamma} \leftarrow \sum_{\delta \in A} \sum_{w \in D} \frac{1}{4} {}^2D^2_{i,w} \tau^7_{\delta,i} \tau^{11}_{\delta,\gamma,w} \tau^{12}_{\delta,\gamma,w} \quad (4r_D r_T^2 N_o) \quad (5467)$$

Factorized expression

Raw expression

$$\tau^0_{\gamma,\alpha} = \sum_{a \in V} W^2_{a,\alpha} Y^1_{a,\gamma} \quad (2r_T r_V N_v) \quad (5454)$$

$${}^2R^2_{i,\epsilon} \leftarrow \sum_{\gamma \in A} \sum_{j \in O} \sum_{k \in O} \sum_{l \in O} \sum_{a \in V} \sum_{b \in V} \sum_{c \in V} \sum_{d \in V} \frac{1}{4} Y^{1,*}_{a,\epsilon} Z^*_{\epsilon,\gamma} Y^{3,*}_{b,\gamma} Y^{4,*}_{j,\gamma} {}^2D^{a,i,b,j} {}^2T_{b,j,a,l} {}^2T_{c,k,d,i} V_{l,c,k,d} \quad (5468)$$

$$\tau^1_{\gamma,\alpha,i} = \sum_{\beta \in B} W^1_{i,\beta} X_{\beta,\alpha} \tau^0_{\gamma,\beta} \quad (3r_T r_V^2 N_o) \quad (5455)$$

Factorized expression

$$\tau^2_{\gamma,\alpha} = \sum_{i \in O} W^3_{i,\alpha} Y^2_{i,\gamma} \quad (2r_T r_V N_o) \quad (5456)$$

$$\tau^0_{\gamma,\alpha} = \sum_{a \in V} W^2_{a,\alpha} Y^1_{a,\gamma} \quad (2r_T r_V N_v) \quad (5469)$$

Factorized expression

$$\tau^1_{\gamma,\alpha,i} = \sum_{\beta \in B} W^1_{i,\beta} X_{\beta,\alpha} \tau^0_{\gamma,\beta} \quad (3r_T r_V^2 N_o) \quad (5470)$$

$$\tau^2_{\gamma,\alpha} = \sum_{a \in V} W^4_{a,\alpha} Y^3_{a,\gamma} \quad (2r_T r_V N_v) \quad (5471)$$

$$\tau^3_{\gamma,\alpha,i} = \sum_{\delta \in A} Z_{\gamma,\delta} Y^4_{i,\delta} \tau^2_{\delta,\alpha} \quad (3r_T^2 r_V N_o) \quad (5472)$$

$$\tau^4_{\gamma,i,j,k} = \sum_{\alpha \in B} W^3_{j,\alpha} \tau^1_{\gamma,\alpha,i} \tau^3_{\gamma,\alpha,k} \quad (3r_T r_V N_o^3) \quad (5473)$$

$$\tau^5_{i,j,k,l} = \sum_{\gamma \in A} Y^2_{k,\gamma} \tau^4_{\gamma,i,j,l} \quad (2r_T N_o^4) \quad (5474)$$

$$\tau^6_{\gamma,i,j,k} = \sum_{l \in O} Y^2_{l,\gamma} \tau^5_{l,i,j,k} \quad (2r_T N_o^4) \quad (5475)$$

$$\tau^7_{\gamma,\delta,w} = \sum_{a \in V} {}^2D^3_{a,w} Y^1_{a,\gamma} Y^{3,*}_{a,\delta} \quad (3r_D r_T^2 N_v) \quad (5476)$$

$$\tau^8_{\gamma,\delta,w,i} = \sum_{\epsilon \in A} Z^*_{\delta,\epsilon} Y^{4,*}_{i,\epsilon} \tau^7_{\gamma,\epsilon,w} \quad (3r_D r_T^3 N_o) \quad (5477)$$

$$\tau^9_{\gamma,\delta,w} = \sum_{a \in V} {}^2D^1_{a,w} Y^3_{a,\gamma} Y^{1,*}_{a,\delta} \quad (3r_D r_T^2 N_v) \quad (5478)$$

$$\tau^{10}_{\gamma,\delta,w,i} = \sum_{\epsilon \in A} Z_{\gamma,\epsilon} Y^4_{i,\epsilon} \tau^9_{\epsilon,\delta,w} \quad (3r_D r_T^3 N_o) \quad (5479)$$

$$\tau^{11}_{\gamma,w,i,j} = \sum_{\delta \in A} \sum_{k \in O} \tau^{10}_{\delta,\gamma,w,k} \tau^6_{\delta,k,i,j} \tau^8_{\delta,\gamma,w,i} \quad (3r_D r_T^2 N_o^3) \quad (5480)$$

$${}^2R^2_{i,\gamma} \leftarrow \sum_{w \in D} \sum_{j \in O} \frac{1}{4} {}^2D^2_{i,w} {}^2D^4_{j,w} \tau^{11}_{\gamma,w,j,i} \quad (3r_D r_T N_o^2) \quad (5481)$$

Raw expression

$${}^2R^2_{i,\epsilon} \leftarrow \sum_{\gamma \in A} \sum_{j \in O} \sum_{k \in O} \sum_{l \in O} \sum_{a \in V} \sum_{b \in V} \sum_{c \in V} \sum_{d \in V} \frac{1}{4} Y^{1,*}_{a,\epsilon} Z^*_{\epsilon,\gamma} Y^{3,*}_{b,\gamma} Y^{4,*}_{j,\gamma} {}^2D^{a,i,b,j} {}^2T_{b,j,c,i} {}^2T_{d,k,a,l} V_{k,c,l,d} \quad (5482)$$

$$\tau^0_{\gamma,\delta,w} = \sum_{a \in V} {}^2D^1_{a,w} Y^3_{a,\gamma} Y^{1,*}_{a,\delta} \quad (3r_D r_T^2 N_v) \quad (5483)$$

$$\tau^1_{\gamma,\alpha} = \sum_{a \in V} W^2_{a,\alpha} Y^1_{a,\gamma} \quad (2r_T r_V N_v) \quad (5484)$$

$$\tau^2_{\gamma,\alpha,i} = \sum_{\beta \in B} W^1_{i,\beta} X_{\beta,\alpha} \tau^1_{\gamma,\beta} \quad (3r_T r_V^2 N_o) \quad (5485)$$

$$\tau^3_{\gamma,\alpha} = \sum_{i \in O} W^3_{i,\alpha} Y^2_{i,\gamma} \quad (2r_T r_V N_o) \quad (5486)$$

$$\tau^4_{\gamma,\alpha} = \sum_{a \in V} W^4_{a,\alpha} Y^3_{a,\gamma} \quad (2r_T r_V N_v) \quad (5487)$$

$$\tau^5_{\gamma,\delta,i} = \sum_{\alpha \in B} \tau^3_{\gamma,\alpha} \tau^4_{\delta,\alpha} \tau^2_{\gamma,\alpha,i} \quad (3r_T^2 r_V N_o) \quad (5488)$$

$$\tau^6_{\gamma,i} = \sum_{\delta \in A} Z_{\delta,\gamma} \tau^5_{\delta,\gamma,i} \quad (2r_T^2 N_o) \quad (5489)$$

$$\tau^7_{i,j} = \sum_{\gamma \in A} Y^4_{j,\gamma} \tau^6_{\gamma,i} \quad (2r_T N_o^2) \quad (5490)$$

$$\tau^8_{\gamma,i} = \sum_{j \in O} Y^2_{j,\gamma} \tau^7_{j,i} \quad (2r_T N_o^2) \quad (5491)$$

$$\tau^9_{\gamma,\delta,w} = \sum_{i \in O} {}^2D^4_{i,w} Y^{4,*}_{i,\delta} \tau^8_{\gamma,i} \quad (3r_D r_T^2 N_o) \quad (5492)$$

$$\tau^{10}_{\gamma,\delta,w} = \sum_{a \in V} {}^2D^3_{a,w} Y^1_{a,\gamma} Y^{3,*}_{a,\delta} \quad (3r_D r_T^2 N_v) \quad (5493)$$

$$\tau^{11}_{\gamma,\delta,w} = \sum_{\epsilon \in A} Z^*_{\delta,\epsilon} \tau^{10}_{\gamma,\epsilon,w} \tau^9_{\gamma,\epsilon,w} \quad (3r_D r_T^3) \quad (5494)$$

$$\tau^{12}_{\gamma,\delta,w} = \sum_{\epsilon \in A} Z_{\epsilon,\gamma} \tau^{11}_{\epsilon,\delta,w} \quad (2r_D r_T^3) \quad (5495)$$

$${}^2R^2_{i,\gamma} \leftarrow \sum_{\delta \in A} \sum_{w \in D} \frac{1}{4} {}^2D^2_{i,w} Y^4_{i,\delta} \tau^0_{\delta,\gamma,w} \tau^{12}_{\delta,\gamma,w} \quad (4r_D r_T^2 N_o) \quad (5496)$$

Raw expression

$${}^2R^2_{i,\epsilon} \leftarrow \sum_{\gamma \in A} \sum_{j \in O} \sum_{k \in O} \sum_{l \in O} \sum_{a \in V} \sum_{b \in V} \sum_{c \in V} \sum_{d \in V} \frac{1}{4} Y^{1,*}_{a,\epsilon} Z^*_{\epsilon,\gamma} Y^{3,*}_{b,\gamma} Y^{4,*}_{j,\gamma} {}^2D^{a,i,b,j} {}^2T_{b,j,d,l} {}^2T_{c,i,a,k} V_{k,d,l,c} \quad (5497)$$

Factorized expression

$$\tau^0_{\gamma,\delta,w} = \sum_{a \in V} {}^2D^3_{a,w} Y^1_{a,\gamma} Y^{3,*}_{a,\delta} (3r_D r_T^2 N_v) \quad (5498)$$

$$\tau^1_{\gamma,\delta,w} = \sum_{i \in O} {}^2D^4_{i,w} Y^2_{i,\gamma} Y^{4,*}_{i,\delta} (3r_D r_T^2 N_o) \quad (5499)$$

$$\tau^2_{\gamma,\delta,w} = \sum_{\epsilon \in A} Z^*_{\delta,\epsilon} \tau^0_{\gamma,\epsilon,w} \tau^1_{\gamma,\epsilon,w} (3r_D r_T^3) \quad (5500)$$

$$\tau^3_{\gamma,\delta,w} = \sum_{\epsilon \in A} Z_{\epsilon,\gamma} \tau^2_{\epsilon,\delta,w} (2r_D r_T^3) \quad (5501)$$

$$\tau^4_{\gamma,\alpha} = \sum_{a \in V} W^4_{a,\alpha} Y^1_{a,\gamma} (2r_T r_V N_v) \quad (5502)$$

$$\tau^5_{\gamma,\alpha,i} = \sum_{\beta \in B} X_{\alpha,\beta} W^3_{i,\beta} \tau^4_{\gamma,\beta} (3r_T r_V^2 N_o) \quad (5503)$$

$$\tau^6_{\gamma,\alpha} = \sum_{i \in O} W^1_{i,\alpha} Y^2_{i,\gamma} (2r_T r_V N_o) \quad (5504)$$

$$\tau^7_{\gamma,\alpha} = \sum_{\delta \in A} \sum_{i \in O} Z_{\delta,\gamma} Y^4_{i,\gamma} \tau^6_{\delta,\alpha} \tau^5_{\delta,\alpha,i} (4r_T^2 r_V N_o) \quad (5505)$$

$$\tau^8_{\gamma,a} = \sum_{\alpha \in B} W^2_{a,\alpha} \tau^7_{\gamma,\alpha} (2r_T r_V N_v) \quad (5506)$$

$$\tau^9_{a,b} = \sum_{\gamma \in A} Y^3_{b,\gamma} \tau^8_{\gamma,a} (2r_T N_v^2) \quad (5507)$$

$$\tau^{10}_{\gamma,a} = \sum_{b \in V} Y^3_{b,\gamma} \tau^9_{b,a} (2r_T N_v^2) \quad (5508)$$

$$\tau^{11}_{\gamma,\delta,w} = \sum_{a \in V} {}^2D^1_{a,w} Y^{1,*}_{a,\delta} \tau^{10}_{\gamma,a} (3r_D r_T^2 N_v) \quad (5509)$$

$${}^2R^2_{i,\gamma} \leftarrow \sum_{\delta \in A} \sum_{w \in D} \frac{1}{4} {}^2D^2_{i,w} Y^4_{i,\delta} \tau^{11}_{\delta,\gamma,w} \tau^3_{\delta,\gamma,w} (4r_D r_T^2 N_o) \quad (5510)$$

Raw expression

$${}^2R^2_{i,\epsilon} \leftarrow \sum_{\gamma \in A} \sum_{j \in O} \sum_{k \in O} \sum_{l \in O} \sum_{a \in V} \sum_{b \in V} \sum_{c \in V} \sum_{d \in V} \frac{1}{4} Y^{1,*}_{a,\epsilon} Z^*_{\epsilon,\gamma} Y^{3,*}_{b,\gamma} Y^{4,*}_{j,\gamma} {}^2D^{a,i,b,j} {}^2T_{b,k,a,i} {}^2T_{c,j,d,l} V_{k,d,l,c} \quad (5511)$$

Factorized expression

$$\tau^0_{\gamma,\delta,w} = \sum_{a \in V} {}^2D^1_{a,w} Y^3_{a,\gamma} Y^{1,*}_{a,\delta} (3r_D r_T^2 N_v) \quad (5512)$$

$$\tau^1_{\gamma,\delta,w} = \sum_{i \in O} {}^2D^4_{i,w} Y^2_{i,\gamma} Y^{4,*}_{i,\delta} (3r_D r_T^2 N_o) \quad (5513)$$

$$\tau^2_{\gamma,\alpha} = \sum_{a \in V} W^2_{a,\alpha} Y^3_{a,\gamma} (2r_T r_V N_v) \quad (5514)$$

$$\tau^3_{\gamma,\alpha,i} = \sum_{\beta \in B} W^1_{i,\beta} X_{\beta,\alpha} \tau^2_{\gamma,\beta} (3r_T r_V^2 N_o) \quad (5515)$$

$$\tau^4_{\gamma,\alpha} = \sum_{i \in O} W^3_{i,\alpha} Y^4_{i,\gamma} (2r_T r_V N_o) \quad (5516)$$

$$\tau^5_{\gamma,\alpha} = \sum_{\delta \in A} \sum_{i \in O} Y^2_{i,\gamma} Z_{\gamma,\delta} \tau^4_{\delta,\alpha} \tau^3_{\delta,\alpha,i} (4r_T^2 r_V N_o) \quad (5517)$$

$$\tau^6_{\gamma,a} = \sum_{\alpha \in B} W^4_{a,\alpha} \tau^5_{\gamma,\alpha} (2r_T r_V N_v) \quad (5518)$$

$$\tau^7_{\gamma,\delta} = \sum_{a \in V} Y^1_{a,\gamma} \tau^6_{\delta,a} (2r_T^2 N_v) \quad (5519)$$

$$\tau^8_{\gamma,a} = \sum_{\delta \in A} Y^1_{a,\delta} \tau^7_{\gamma,\delta} (2r_T^2 N_v) \quad (5520)$$

$$\tau^9_{\gamma,\delta,w} = \sum_{a \in V} {}^2D^3_{a,w} Y^{3,*}_{a,\delta} \tau^8_{\gamma,a} (3r_D r_T^2 N_v) \quad (5521)$$

$$\tau^{10}_{\gamma,\delta,w} = \sum_{\epsilon \in A} Z^*_{\delta,\epsilon} \tau^1_{\gamma,\epsilon,w} \tau^9_{\gamma,\epsilon,w} (3r_D r_T^3) \quad (5522)$$



$$\tau^{11}_{\gamma,\delta,w} = \sum_{\epsilon \in A} Z_{\epsilon,\gamma} \tau^{10}_{\epsilon,\delta,w} \quad (2r_D r_T^3) \quad (5523)$$

$$\tau^{10}_{\gamma,\delta,w} = \sum_{a \in V} {}^2D^3_{a,w} Y^1_{a,\gamma} Y^{3,*}_{a,\delta} \quad (3r_D r_T^2 N_v) \quad (5536)$$

$${}^2R^2_{i,\gamma} \leftarrow \sum_{\delta \in A} \sum_{w \in D} \frac{1}{4} {}^2D^2_{i,w} Y^4_{i,\delta} \tau^0_{\delta,\gamma,w} \tau^{11}_{\delta,\gamma,w} \quad (4r_D r_T^2 N_o) \quad (5524)$$

$$\tau^{11}_{\gamma,\delta,w} = \sum_{\epsilon \in A} Z^*_{\delta,\epsilon} \tau^{10}_{\gamma,\epsilon,w} \tau^9_{\gamma,\epsilon,w} \quad (3r_D r_T^3) \quad (5537)$$

Raw expression

$${}^2R^2_{i,\epsilon} \leftarrow \sum_{\gamma \in A} \sum_{j \in O} \sum_{k \in O} \sum_{l \in O} \sum_{a \in V} \sum_{b \in V} \sum_{c \in V} \sum_{d \in V} \frac{1}{4} Y^{1,*}_{a,\epsilon} Z^*_{\epsilon,\gamma} Y^{3,*}_{b,\gamma} Y^{4,*}_{j,\gamma} {}^2D^{a,i,b,j} {}^2T_{b,k,a,i} {}^2T_{c,l,d,j} V_{k,c,l,d} \quad (5525)$$

$$\tau^{12}_{\gamma,\delta,w} = \sum_{\epsilon \in A} Z_{\epsilon,\gamma} \tau^{11}_{\epsilon,\delta,w} \quad (2r_D r_T^3) \quad (5538)$$

$${}^2R^2_{i,\gamma} \leftarrow \sum_{\delta \in A} \sum_{w \in D} \frac{1}{4} {}^2D^2_{i,w} Y^4_{i,\delta} \tau^0_{\delta,\gamma,w} \tau^{12}_{\delta,\gamma,w} \quad (4r_D r_T^2 N_o) \quad (5539)$$

Factorized expression

$$\tau^0_{\gamma,\delta,w} = \sum_{a \in V} {}^2D^1_{a,w} Y^3_{a,\gamma} Y^{1,*}_{a,\delta} \quad (3r_D r_T^2 N_v) \quad (5526)$$

Raw expression

$${}^2R^2_{i,\epsilon} \leftarrow \sum_{\gamma \in A} \sum_{j \in O} \sum_{k \in O} \sum_{l \in O} \sum_{a \in V} \sum_{b \in V} \sum_{c \in V} \sum_{d \in V} \frac{1}{4} Y^{1,*}_{a,\epsilon} Z^*_{\epsilon,\gamma} Y^{3,*}_{b,\gamma} Y^{4,*}_{j,\gamma} {}^2D^{a,i,b,j} {}^2T_{b,k,a,l} {}^2T_{c,i,d,j} V_{k,d,l,c} \quad (5540)$$

$$\tau^1_{\gamma,\alpha} = \sum_{a \in V} W^2_{a,\alpha} Y^3_{a,\gamma} \quad (2r_T r_V N_v) \quad (5527)$$

Factorized expression

$$\tau^2_{\gamma,\alpha,i} = \sum_{\beta \in B} W^1_{i,\beta} X_{\beta,\alpha} \tau^1_{\gamma,\beta} \quad (3r_T r_V^2 N_o) \quad (5528)$$

$$\tau^0_{\gamma,\alpha} = \sum_{a \in V} W^2_{a,\alpha} Y^3_{a,\gamma} \quad (2r_T r_V N_v) \quad (5541)$$

$$\tau^3_{\gamma,\alpha} = \sum_{i \in O} W^3_{i,\alpha} Y^4_{i,\gamma} \quad (2r_T r_V N_o) \quad (5529)$$

$$\tau^1_{\gamma,\alpha,i} = \sum_{\delta \in A} Z_{\gamma,\delta} Y^4_{i,\delta} \tau^0_{\delta,\alpha} \quad (3r_T^2 r_V N_o) \quad (5542)$$

$$\tau^4_{\gamma,\alpha} = \sum_{a \in V} W^4_{a,\alpha} Y^1_{a,\gamma} \quad (2r_T r_V N_v) \quad (5530)$$

$$\tau^2_{\gamma,\delta,w} = \sum_{a \in V} {}^2D^3_{a,w} Y^1_{a,\gamma} Y^{3,*}_{a,\delta} \quad (3r_D r_T^2 N_v) \quad (5543)$$

$$\tau^5_{\gamma,\delta,i} = \sum_{\alpha \in B} \tau^3_{\delta,\alpha} \tau^4_{\gamma,\alpha} \tau^2_{\delta,\alpha,i} \quad (3r_T^2 r_V N_o) \quad (5531)$$

$$\tau^3_{\gamma,\delta,w,i} = \sum_{\epsilon \in A} Z^*_{\delta,\epsilon} Y^{4,*}_{i,\epsilon} \tau^2_{\gamma,\epsilon,w} \quad (3r_D r_T^3 N_o) \quad (5544)$$

$$\tau^6_{\gamma,i} = \sum_{\delta \in A} Z_{\gamma,\delta} \tau^5_{\gamma,\delta,i} \quad (2r_T^2 N_o) \quad (5532)$$

$$\tau^4_{\gamma,\delta,\epsilon,w} = \sum_{i \in O} {}^2D^4_{i,w} Y^2_{i,\delta} \tau^3_{\gamma,\epsilon,w,i} \quad (3r_D r_T^3 N_o) \quad (5545)$$

$$\tau^7_{i,j} = \sum_{\gamma \in A} Y^2_{j,\gamma} \tau^6_{\gamma,i} \quad (2r_T N_o^2) \quad (5533)$$

$$\tau^5_{\gamma,\delta,w} = \sum_{a \in V} {}^2D^1_{a,w} Y^3_{a,\gamma} Y^{1,*}_{a,\delta} \quad (3r_D r_T^2 N_v) \quad (5546)$$

$$\tau^8_{\gamma,i} = \sum_{j \in O} Y^2_{j,\gamma} \tau^7_{j,i} \quad (2r_T N_o^2) \quad (5534)$$

$$\tau^6_{\gamma,\delta,w,i} = \sum_{\epsilon \in A} Z_{\gamma,\epsilon} Y^4_{i,\epsilon} \tau^5_{\epsilon,\delta,w} \quad (3r_D r_T^3 N_o) \quad (5547)$$

$$\tau^9_{\gamma,\delta,w} = \sum_{i \in O} {}^2D^4_{i,w} Y^{4,*}_{i,\delta} \tau^8_{\gamma,i} \quad (3r_D r_T^2 N_o) \quad (5535)$$

$$\tau^7_{\gamma,\delta,\alpha,w} = \sum_{i \in O} W^1_{i,\alpha} \tau^6_{\gamma,\delta,w,i} \quad (2r_D r_T^2 r_V N_o) \quad (5548)$$

$$\tau^8_{\gamma,\alpha} = \sum_{a \in V} W^4_{a,\alpha} Y^1_{a,\gamma} \quad (2r_T r_V N_v) \quad (5549)$$

$$\tau^6_{\gamma,\delta,i} = \sum_{\alpha \in B} \tau^4_{\gamma,\alpha} \tau^5_{\delta,\alpha} \tau^3_{\gamma,\alpha,i} \quad (3r_T^2 r_V N_o) \quad (5562)$$

$$\tau^9_{\gamma,\alpha,i} = \sum_{\beta \in B} X_{\alpha,\beta} W^3_{i,\beta} \tau^8_{\gamma,\beta} \quad (3r_T r_V^2 N_o) \quad (5550)$$

$$\tau^7_{\gamma,\delta,\epsilon} = \sum_{i \in O} Y^2_{i,\delta} Z_{\delta,\epsilon} \tau^6_{\gamma,\epsilon,i} \quad (3r_T^3 N_o) \quad (5563)$$

$$\tau^{10}_{\gamma,\delta,\alpha} = \sum_{i \in O} Y^2_{i,\delta} \tau^9_{\gamma,\alpha,i} \quad (2r_T^2 r_V N_o) \quad (5551)$$

$$\tau^8_{\gamma,\delta,i} = \sum_{\epsilon \in A} Y^4_{i,\epsilon} \tau^7_{\gamma,\delta,\epsilon} \quad (2r_T^3 N_o) \quad (5564)$$

$$\tau^{11}_{\gamma,\delta,\alpha,w} = \sum_{\epsilon \in A} \tau^{10}_{\epsilon,\gamma,\alpha} \tau^4_{\gamma,\epsilon,\delta,w} \tau^7_{\epsilon,\delta,\alpha,w} \quad (3r_D r_T^3 r_V) \quad (5552)$$

$$\tau^9_{\gamma,\delta,w} = \sum_{\epsilon \in A} \sum_{i \in O} {}^2D^4_{i,w} Y^{4,*}_{i,\delta} \tau^1_{\epsilon,\delta,w} \tau^8_{\gamma,\epsilon,i} \quad (4r_D r_T^3 N_o) \quad (5565)$$

$$\tau^{12}_{\gamma,w,i} = \sum_{\delta \in A} \sum_{\alpha \in B} \tau^1_{\delta,\alpha,i} \tau^{11}_{\delta,\gamma,\alpha,w} \quad (2r_D r_T^2 r_V N_o) \quad (5553)$$

$$\tau^{10}_{\gamma,\delta,w} = \sum_{\epsilon \in A} Z^*_{\delta,\epsilon} \tau^9_{\gamma,\epsilon,w} \quad (2r_D r_T^3) \quad (5566)$$

$${}^2R^2_{i,\gamma} \leftarrow \sum_{w \in D} \frac{1}{4} {}^2D^2_{i,w} \tau^{12}_{\gamma,w,i} \quad (2r_D r_T N_o) \quad (5554)$$

$$\tau^{11}_{\gamma,\delta,w} = \sum_{\epsilon \in A} Z_{\epsilon,\gamma} \tau^{10}_{\epsilon,\delta,w} \quad (2r_D r_T^3) \quad (5567)$$

Raw expression

$${}^2R^2_{i,\epsilon} \leftarrow \sum_{\gamma \in A} \sum_{j \in O} \sum_{k \in O} \sum_{l \in O} \sum_{a \in V} \sum_{b \in V} \sum_{c \in V} \sum_{d \in V} \frac{1}{4} Y^{1,*}_{a,\epsilon} Z^*_{\epsilon,\gamma} Y^{3,*}_{b,\gamma} Y^{4,*}_{j,\gamma} {}^2D^{a,i,b,j} {}^2T_{b,k,a,l} {}^2T_{c,j,d,i} V_{k,c,l,d} \quad (5555)$$

Factorized expression

$$\tau^0_{\gamma,\delta,w} = \sum_{a \in V} {}^2D^1_{a,w} Y^3_{a,\gamma} Y^{1,*}_{a,\delta} \quad (3r_D r_T^2 N_v) \quad (5556)$$

$${}^2R^2_{i,\gamma} \leftarrow \sum_{\delta \in A} \sum_{w \in D} \frac{1}{4} {}^2D^2_{i,w} Y^4_{i,\delta} \tau^0_{\delta,\gamma,w} \tau^{11}_{\delta,\gamma,w} \quad (4r_D r_T^2 N_o) \quad (5568)$$

Raw expression

$${}^2R^2_{i,\epsilon} \leftarrow \sum_{\gamma \in A} \sum_{j \in O} \sum_{k \in O} \sum_{l \in O} \sum_{a \in V} \sum_{b \in V} \sum_{c \in V} \sum_{d \in V} \frac{1}{4} Y^{1,*}_{a,\epsilon} Z^*_{\epsilon,\gamma} Y^{3,*}_{b,\gamma} Y^{4,*}_{j,\gamma} {}^2D^{a,i,b,j} {}^2T_{b,k,c,i} {}^2T_{d,j,a,l} V_{l,c,k,d} \quad (5569)$$

Factorized expression

$$\tau^1_{\gamma,\delta,w} = \sum_{a \in V} {}^2D^3_{a,w} Y^1_{a,\gamma} Y^{3,*}_{a,\delta} \quad (3r_D r_T^2 N_v) \quad (5557)$$

$$\tau^0_{\gamma,\delta,w} = \sum_{a \in V} {}^2D^1_{a,w} Y^3_{a,\gamma} Y^{1,*}_{a,\delta} \quad (3r_D r_T^2 N_v) \quad (5570)$$

$$\tau^2_{\gamma,\alpha} = \sum_{a \in V} W^4_{a,\alpha} Y^1_{a,\gamma} \quad (2r_T r_V N_v) \quad (5558)$$

$$\tau^1_{\gamma,\alpha} = \sum_{a \in V} W^2_{a,\alpha} Y^1_{a,\gamma} \quad (2r_T r_V N_v) \quad (5571)$$

$$\tau^3_{\gamma,\alpha,i} = \sum_{\beta \in B} X_{\alpha,\beta} W^3_{i,\beta} \tau^2_{\gamma,\beta} \quad (3r_T r_V^2 N_o) \quad (5559)$$

$$\tau^2_{\gamma,\alpha,i} = \sum_{\delta \in A} Y^2_{i,\delta} Z_{\delta,\gamma} \tau^1_{\delta,\alpha} \quad (3r_T^2 r_V N_o) \quad (5572)$$

$$\tau^4_{\gamma,\alpha} = \sum_{i \in O} W^1_{i,\alpha} Y^2_{i,\gamma} \quad (2r_T r_V N_o) \quad (5560)$$

$$\tau^3_{\gamma,\alpha} = \sum_{i \in O} W^1_{i,\alpha} Y^4_{i,\gamma} \quad (2r_T r_V N_o) \quad (5573)$$

$$\tau^5_{\gamma,\alpha} = \sum_{a \in V} W^2_{a,\alpha} Y^3_{a,\gamma} \quad (2r_T r_V N_v) \quad (5561)$$

$$\tau^4_{\gamma,\delta,w} = \sum_{a \in V} {}^2D^3_{a,w} Y^1_{a,\gamma} Y^{3,*}_{a,\delta} \quad (3r_D r_T^2 N_v) \quad (5574)$$

$$\tau^5_{\gamma,\alpha} = \sum_{i \in O} W^3_{i,\alpha} Y^2_{i,\gamma} \quad (2r_T r_V N_o) \quad (5575)$$

$$\tau^3_{\gamma,\alpha} = \sum_{a \in V} W^4_{a,\alpha} Y^1_{a,\gamma} \quad (2r_T r_V N_v) \quad (5588)$$

$$\tau^6_{\gamma,\alpha} = \sum_{a \in V} W^4_{a,\alpha} Y^3_{a,\gamma} \quad (2r_T r_V N_v) \quad (5576)$$

$$\tau^4_{\gamma,\delta,i} = \sum_{\alpha \in B} \tau^2_{\delta,\alpha} \tau^3_{\gamma,\alpha} \tau^1_{\delta,\alpha,i} \quad (3r_T^2 r_V N_o) \quad (5589)$$

$$\tau^7_{\gamma,\alpha,i} = \sum_{\delta \in A} Z_{\gamma,\delta} Y^4_{i,\delta} \tau^6_{\delta,\alpha} \quad (3r_T^2 r_V N_o) \quad (5577)$$

$$\tau^5_{\gamma,i} = \sum_{\delta \in A} Z_{\gamma,\delta} \tau^4_{\gamma,\delta,i} \quad (2r_T^2 N_o) \quad (5590)$$

$$\tau^8_{\gamma,\alpha,w} = \sum_{\delta \in A} \sum_{i \in O} {}^2D^4_{i,w} Y^{4,*}_{i,\gamma} \tau^5_{\delta,\alpha} \tau^4_{\delta,\gamma,w} \tau^7_{\delta,\alpha,i} \quad (5r_D r_T^2 r_V N_o) \quad (5578)$$

$$\tau^6_{i,j} = \sum_{\gamma \in A} Y^2_{j,\gamma} \tau^5_{\gamma,i} \quad (2r_T N_o^2) \quad (5591)$$

$$\tau^9_{\gamma,\alpha,w} = \sum_{\beta \in B} X_{\alpha,\beta} \tau^8_{\gamma,\beta,w} \quad (2r_D r_T r_V^2) \quad (5579)$$

$$\tau^7_{\gamma,i} = \sum_{j \in O} Y^4_{j,\gamma} \tau^6_{j,i} \quad (2r_T N_o^2) \quad (5592)$$

$$\tau^{10}_{\gamma,\alpha,w} = \sum_{\delta \in A} Z^*_{\gamma,\delta} \tau^9_{\delta,\alpha,w} \quad (2r_D r_T^2 r_V) \quad (5580)$$

$$\tau^8_{\gamma,\delta,w} = \sum_{a \in V} {}^2D^3_{a,w} Y^1_{a,\gamma} Y^{3,*}_{a,\delta} \quad (3r_D r_T^2 N_v) \quad (5593)$$

$$\tau^{11}_{\gamma,\delta,w,i} = \sum_{\alpha \in B} \tau^3_{\gamma,\alpha} \tau^{10}_{\delta,\alpha,w} \tau^2_{\gamma,\alpha,i} \quad (3r_D r_T^2 r_V N_o) \quad (5581)$$

$$\tau^9_{\gamma,\delta,w} = \sum_{i \in O} {}^2D^4_{i,w} Y^2_{i,\gamma} Y^{4,*}_{i,\delta} \quad (3r_D r_T^2 N_o) \quad (5594)$$

$$\tau^{10}_{\gamma,\delta,w} = \sum_{\epsilon \in A} Z^*_{\delta,\epsilon} \tau^8_{\gamma,\epsilon,w} \tau^9_{\gamma,\epsilon,w} \quad (3r_D r_T^3) \quad (5595)$$

$$\tau^{12}_{\gamma,w,i} = \sum_{\delta \in A} \tau^0_{\delta,\gamma,w} \tau^{11}_{\delta,\gamma,w,i} \quad (2r_D r_T^2 N_o) \quad (5582)$$

$$\tau^{11}_{\gamma,\delta,w} = \sum_{\epsilon \in A} Z_{\epsilon,\gamma} \tau^{10}_{\epsilon,\delta,w} \quad (2r_D r_T^3) \quad (5596)$$

$${}^2R^2_{i,\gamma} \leftarrow \sum_{w \in D} \frac{1}{4} {}^2D^2_{i,w} \tau^{12}_{\gamma,w,i} \quad (2r_D r_T N_o) \quad (5583)$$

$$\tau^{12}_{\gamma,\delta,w} = \sum_{a \in V} {}^2D^1_{a,w} Y^3_{a,\gamma} Y^{1,*}_{a,\delta} \quad (3r_D r_T^2 N_v) \quad (5597)$$

Raw expression

$${}^2R^2_{i,\epsilon} \leftarrow \sum_{\gamma \in A} \sum_{j \in O} \sum_{k \in O} \sum_{l \in O} \sum_{a \in V} \sum_{b \in V} \sum_{c \in V} \sum_{d \in V} \frac{1}{4} Y^{1,*}_{a,\epsilon} Z^*_{\epsilon,\gamma} Y^{3,*}_{b,\gamma} Y^{4,*}_{j,\gamma} {}^2D^{a,i,b,j} {}^2T_{b,k,d,l} {}^2T_{c,j,a,i} V_{k,d,l,c} \quad (5584)$$

$${}^2R^2_{i,\gamma} \leftarrow \sum_{\delta \in A} \sum_{w \in D} \frac{1}{4} {}^2D^2_{i,w} \tau^7_{\delta,i} \tau^{11}_{\delta,\gamma,w} \tau^{12}_{\delta,\gamma,w} \quad (4r_D r_T^2 N_o) \quad (5598)$$

Factorized expression

$$\tau^0_{\gamma,\alpha} = \sum_{a \in V} W^2_{a,\alpha} Y^3_{a,\gamma} \quad (2r_T r_V N_v) \quad (5585)$$

Raw expression

$${}^2R^2_{i,\epsilon} \leftarrow \sum_{\gamma \in A} \sum_{j \in O} \sum_{k \in O} \sum_{l \in O} \sum_{a \in V} \sum_{b \in V} \sum_{c \in V} \sum_{d \in V} \frac{1}{4} Y^{1,*}_{a,\epsilon} Z^*_{\epsilon,\gamma} Y^{3,*}_{b,\gamma} Y^{4,*}_{j,\gamma} {}^2D^{a,i,b,j} {}^2T_{b,l,d,j} {}^2T_{c,i,a,k} V_{k,c,l,d} \quad (5599)$$

$$\tau^1_{\gamma,\alpha,i} = \sum_{\beta \in B} W^1_{i,\beta} X_{\beta,\alpha} \tau^0_{\gamma,\beta} \quad (3r_T r_V^2 N_o) \quad (5586)$$

Factorized expression

$$\tau^2_{\gamma,\alpha} = \sum_{i \in O} W^3_{i,\alpha} Y^4_{i,\gamma} \quad (2r_T r_V N_o) \quad (5587)$$

$$\tau^0_{\gamma,\delta,w} = \sum_{a \in V} {}^2D^1_{a,w} Y^3_{a,\gamma} Y^{1,*}_{a,\delta} \quad (3r_D r_T^2 N_v) \quad (5600)$$

$$\tau^1_{\gamma,\delta,w} = \sum_{a \in V} {}^2D^3_{a,w} Y^1_{a,\gamma} Y^{3,*}_{a,\delta} \quad (3r_D r_T^2 N_v) \quad (5601)$$

$$\tau^2_{\gamma,\delta,w} = \sum_{i \in O} {}^2D^4_{i,w} Y^2_{i,\gamma} Y^{4,*}_{i,\delta} \quad (3r_D r_T^2 N_o) \quad (5602)$$

$$\tau^3_{\gamma,\delta,w} = \sum_{\epsilon \in A} Z^*_{\delta,\epsilon} \tau^1_{\gamma,\epsilon,w} \tau^2_{\gamma,\epsilon,w} \quad (3r_D r_T^3) \quad (5603)$$

$$\tau^4_{\gamma,\delta,w} = \sum_{\epsilon \in A} Z_{\epsilon,\gamma} \tau^3_{\epsilon,\delta,w} \quad (2r_D r_T^3) \quad (5604)$$

$$\tau^5_{\gamma,\alpha} = \sum_{a \in V} W^2_{a,\alpha} Y^3_{a,\gamma} \quad (2r_T r_V N_v) \quad (5605)$$

$$\tau^6_{\gamma,\alpha,i} = \sum_{\beta \in B} W^1_{i,\beta} X_{\beta,\alpha} \tau^5_{\gamma,\beta} \quad (3r_T r_V^2 N_o) \quad (5606)$$

$$\tau^7_{\gamma,\alpha} = \sum_{i \in O} W^3_{i,\alpha} Y^4_{i,\gamma} \quad (2r_T r_V N_o) \quad (5607)$$

$$\tau^8_{\gamma,\alpha} = \sum_{a \in V} W^4_{a,\alpha} Y^1_{a,\gamma} \quad (2r_T r_V N_v) \quad (5608)$$

$$\tau^9_{\gamma,\delta,i} = \sum_{\alpha \in B} \tau^7_{\delta,\alpha} \tau^8_{\gamma,\alpha} \tau^6_{\delta,\alpha,i} \quad (3r_T^2 r_V N_o) \quad (5609)$$

$$\tau^{10}_{\gamma,\delta,\epsilon} = \sum_{i \in O} Z_{\gamma,\delta} Y^4_{i,\delta} \tau^9_{\gamma,\epsilon,i} \quad (3r_T^3 N_o) \quad (5610)$$

$$\tau^{11}_{\gamma,\delta,i} = \sum_{\epsilon \in A} Y^2_{i,\epsilon} \tau^{10}_{\epsilon,\gamma,\delta} \quad (2r_T^3 N_o) \quad (5611)$$

$$\tau^{12}_{\gamma,\delta,w,i} = \sum_{\epsilon \in A} \tau^{11}_{\gamma,\epsilon,i} \tau^4_{\epsilon,\delta,w} \quad (2r_D r_T^3 N_o) \quad (5612)$$

$$\tau^{13}_{\gamma,w,i} = \sum_{\delta \in A} \tau^0_{\delta,\gamma,w} \tau^{12}_{\delta,\gamma,w,i} \quad (2r_D r_T^2 N_o) \quad (5613)$$

$${}^2R^2_{i,\gamma} \leftarrow \sum_{w \in D} \frac{1}{4} {}^2D^2_{i,w} \tau^{13}_{\gamma,w,i} \quad (2r_D r_T N_o) \quad (5614)$$

Raw expression

$${}^2R^2_{i,\epsilon} \leftarrow \sum_{\gamma \in A} \sum_{j \in O} \sum_{k \in O} \sum_{l \in O} \sum_{a \in V} \sum_{b \in V} \sum_{c \in V} \sum_{d \in V} \frac{1}{4} Y^{1,*}_{a,\epsilon} Z^*_{\epsilon,\gamma} Y^{3,*}_{b,\gamma} Y^{4,*}_{j,\gamma} {}^2D^{a,i,b,j} {}^2T_{b,l,d,j} {}^2T_{c,k,a,i} V_{k,d,l,c} \quad (5615)$$

Factorized expression

$$\tau^0_{\gamma,\alpha} = \sum_{a \in V} W^4_{a,\alpha} Y^1_{a,\gamma} \quad (2r_T r_V N_v) \quad (5616)$$

$$\tau^1_{\gamma,\alpha,i} = \sum_{\beta \in B} X_{\alpha,\beta} W^3_{i,\beta} \tau^0_{\gamma,\beta} \quad (3r_T r_V^2 N_o) \quad (5617)$$

$$\tau^2_{\gamma,\alpha} = \sum_{a \in V} W^2_{a,\alpha} Y^3_{a,\gamma} \quad (2r_T r_V N_v) \quad (5618)$$

$$\tau^3_{\gamma,\alpha,i} = \sum_{\delta \in A} Z_{\gamma,\delta} Y^4_{i,\delta} \tau^2_{\delta,\alpha} \quad (3r_T^2 r_V N_o) \quad (5619)$$

$$\tau^4_{\gamma,i,j,k} = \sum_{\alpha \in B} W^1_{i,\alpha} \tau^1_{\gamma,\alpha,j} \tau^3_{\gamma,\alpha,k} \quad (3r_T r_V N_o^3) \quad (5620)$$

$$\tau^5_{i,j,k,l} = \sum_{\gamma \in A} Y^2_{k,\gamma} \tau^4_{\gamma,i,j,l} \quad (2r_T N_o^4) \quad (5621)$$

$$\tau^6_{\gamma,i,j,k} = \sum_{l \in O} Y^2_{l,\gamma} \tau^5_{l,i,j,k} \quad (2r_T N_o^4) \quad (5622)$$

$$\tau^7_{\gamma,\delta,w} = \sum_{a \in V} {}^2D^3_{a,w} Y^1_{a,\gamma} Y^{3,*}_{a,\delta} \quad (3r_D r_T^2 N_v) \quad (5623)$$

$$\tau^8_{\gamma,\delta,w,i} = \sum_{\epsilon \in A} Z^*_{\delta,\epsilon} Y^{4,*}_{i,\epsilon} \tau^7_{\gamma,\epsilon,w} \quad (3r_D r_T^3 N_o) \quad (5624)$$

$$\tau^9_{\gamma,\delta,w} = \sum_{a \in V} {}^2D^1_{a,w} Y^3_{a,\gamma} Y^{1,*}_{a,\delta} \quad (3r_D r_T^2 N_v) \quad (5625)$$

$$\tau^{10}_{\gamma,\delta,w,i} = \sum_{\epsilon \in A} Z_{\gamma,\epsilon} Y^4_{i,\epsilon} \tau^9_{\epsilon,\delta,w} \quad (3r_D r_T^3 N_o) \quad (5626)$$

$$\tau^{11}_{\gamma,w,i,j} = \sum_{\delta \in A} \sum_{k \in O} \tau^{10}_{\delta,\gamma,w,k} \tau^6_{\delta,k,i,j} \tau^8_{\delta,\gamma,w,j} \quad (3r_D r_T^2 N_o^3) \quad (5627)$$

$${}^2R^2_{i,\gamma} \leftarrow \sum_{w \in D} \sum_{j \in O} \frac{1}{4} {}^2D^2_{i,w} {}^2D^4_{j,w} \tau^{11}_{\gamma,w,i,j} \quad (3r_D r_T N_o^2) \quad (5628)$$

Raw expression

$${}^2R^2_{i,\epsilon} \leftarrow \sum_{\gamma \in A} \sum_{j \in O} \sum_{k \in O} \sum_{l \in O} \sum_{a \in V} \sum_{b \in V} \sum_{c \in V} \sum_{d \in V} \frac{1}{4} Y^{1,*}_{a,\epsilon} Z^*_{\epsilon,\gamma} Y^{3,*}_{b,\gamma} Y^{4,*}_{j,\gamma} {}^2D^{a,i,b,j} {}^2T_{c,i,a,k} {}^2T_{d,j,b,l} V_{k,c,l,d} \quad (5629)$$

Factorized expression

$$\tau^0_{\gamma,\alpha} = \sum_{a \in V} W^2_{a,\alpha} Y^1_{a,\gamma} \quad (2r_T r_V N_v) \quad (5630)$$

$$\tau^1_{\gamma,\alpha,i} = \sum_{\delta \in A} Y^2_{i,\delta} Z_{\delta,\gamma} \tau^0_{\delta,\alpha} \quad (3r_T^2 r_V N_o) \quad (5631)$$

$$\tau^2_{\gamma,\delta,w} = \sum_{a \in V} {}^2D^3_{a,w} Y^3_{a,\gamma} Y^{3,*}_{a,\delta} \quad (3r_D r_T^2 N_v) \quad (5632)$$

$$\tau^3_{\gamma,\delta,w,i} = \sum_{\epsilon \in A} Z^*_{\delta,\epsilon} Y^{4,*}_{i,\epsilon} \tau^2_{\gamma,\epsilon,w} \quad (3r_D r_T^3 N_o) \quad (5633)$$

$$\tau^4_{\gamma,\delta,\epsilon,w} = \sum_{i \in O} {}^2D^4_{i,w} Y^2_{i,\gamma} \tau^3_{\delta,\epsilon,w,i} \quad (3r_D r_T^3 N_o) \quad (5634)$$

$$\tau^5_{\gamma,\delta,w} = \sum_{a \in V} {}^2D^1_{a,w} Y^3_{a,\gamma} Y^{1,*}_{a,\delta} \quad (3r_D r_T^2 N_v) \quad (5635)$$

$$\tau^6_{\gamma,\delta,w,i} = \sum_{\epsilon \in A} Z_{\gamma,\epsilon} Y^4_{i,\epsilon} \tau^5_{\epsilon,\delta,w} \quad (3r_D r_T^3 N_o) \quad (5636)$$

$$\tau^7_{\gamma,\delta,\alpha,w} = \sum_{i \in O} W^1_{i,\alpha} \tau^6_{\gamma,\delta,w,i} \quad (2r_D r_T^2 r_V N_o) \quad (5637)$$

$$\tau^8_{\gamma,\alpha} = \sum_{a \in V} W^4_{a,\alpha} Y^1_{a,\gamma} \quad (2r_T r_V N_v) \quad (5638)$$

$$\tau^9_{\gamma,\alpha,i} = \sum_{\beta \in B} X_{\alpha,\beta} W^3_{i,\beta} \tau^8_{\gamma,\beta} \quad (3r_T r_V^2 N_o) \quad (5639)$$

$$\tau^{10}_{\gamma,\delta,\alpha} = \sum_{i \in O} Y^4_{i,\delta} \tau^9_{\gamma,\alpha,i} \quad (2r_T^2 r_V N_o) \quad (5640)$$

$$\tau^{11}_{\gamma,\delta,\alpha,w} = \sum_{\epsilon \in A} \tau^{10}_{\epsilon,\gamma,\alpha} \tau^4_{\epsilon,\gamma,\delta,w} \tau^7_{\epsilon,\delta,\alpha,w} \quad (3r_D r_T^3 r_V) \quad (5641)$$

$$\tau^{12}_{\gamma,w,i} = \sum_{\delta \in A} \sum_{\alpha \in B} \tau^1_{\delta,\alpha,i} \tau^{11}_{\delta,\gamma,\alpha,w} \quad (2r_D r_T^2 r_V N_o) \quad (5642)$$

$${}^2R^2_{i,\gamma} \leftarrow \sum_{w \in D} \frac{1}{4} {}^2D^2_{i,w} \tau^{12}_{\gamma,w,i} \quad (2r_D r_T N_o) \quad (5643)$$

Raw expression

$${}^2R^2_{i,\epsilon} \leftarrow \sum_{\gamma \in A} \sum_{j \in O} \sum_{k \in O} \sum_{l \in O} \sum_{a \in V} \sum_{b \in V} \sum_{c \in V} \sum_{d \in V} \frac{1}{4} Y^{1,*}_{a,\epsilon} Z^*_{\epsilon,\gamma} Y^{3,*}_{b,\gamma} Y^{4,*}_{j,\gamma} {}^2D^{a,i,b,j} {}^2T_{c,i,a,k} {}^2T_{d,l,b,j} V_{k,d,l,c} \quad (5644)$$

Factorized expression

$$\tau^0_{\gamma,\delta,w} = \sum_{a \in V} {}^2D^1_{a,w} Y^3_{a,\gamma} Y^{1,*}_{a,\delta} \quad (3r_D r_T^2 N_v) \quad (5645)$$

$$\tau^1_{\gamma,\delta,w} = \sum_{a \in V} {}^2D^3_{a,w} Y^3_{a,\gamma} Y^{3,*}_{a,\delta} \quad (3r_D r_T^2 N_v) \quad (5646)$$

$$\tau^2_{\gamma,\alpha} = \sum_{a \in V} W^4_{a,\alpha} Y^1_{a,\gamma} \quad (2r_T r_V N_v) \quad (5647)$$

$$\tau^3_{\gamma,\alpha,i} = \sum_{\delta \in A} Y^2_{i,\delta} Z_{\delta,\gamma} \tau^2_{\delta,\alpha} \quad (3r_T^2 r_V N_o) \quad (5648)$$

$$\tau^4_{\gamma,\alpha} = \sum_{i \in O} W^3_{i,\alpha} Y^4_{i,\gamma} \quad (2r_T r_V N_o) \quad (5649)$$

$$\tau^5_{\gamma,\alpha,w} = \sum_{\delta \in A} \sum_{i \in O} {}^2D^4_{i,w} Y^{4,*}_{i,\gamma} \tau^4_{\delta,\alpha} \tau^1_{\delta,\gamma,w} \tau^3_{\delta,\alpha,i} \quad (5r_D r_T^2 r_V N_o) \quad (5650)$$

$$\tau^6_{\gamma,\alpha,w} = \sum_{\beta \in B} X_{\alpha,\beta} \tau^5_{\gamma,\beta,w} \quad (2r_D r_T r_V^2) \quad (5651)$$

$$\tau^7_{\gamma,\alpha,w} = \sum_{\delta \in A} Z^*_{\gamma,\delta} \tau^6_{\delta,\alpha,w} \quad (2r_D r_T^2 r_V) \quad (5652)$$

$$\tau^8_{\gamma,\alpha} = \sum_{a \in V} W^2_{a,\alpha} Y^1_{a,\gamma} \quad (2r_T r_V N_v) \quad (5653)$$

$$\tau_{\gamma,\alpha,i}^9 = \sum_{\delta \in A} Y_{i,\delta}^2 Z_{\delta,\gamma} \tau_{\delta,\alpha}^8 \quad (3r_T^2 r_V N_o) \quad (5654)$$

$$\tau_{\gamma,\delta,w}^7 = \sum_{a \in V} {}^2D_{a,w}^1 Y_{a,\gamma}^{1,*} {}_{a,\delta} \tau_{\gamma,a}^6 \quad (3r_D r_T^2 N_v) \quad (5667)$$

$$\tau_{\gamma,\alpha}^{10} = \sum_{i \in O} W_{i,\alpha}^1 Y_{i,\gamma}^4 \quad (2r_T r_V N_o) \quad (5655)$$

$$\tau_{\gamma,\delta,w}^8 = \sum_{a \in V} {}^2D_{a,w}^3 Y_{a,\gamma}^3 Y_{a,\delta}^{3,*} \quad (3r_D r_T^2 N_v) \quad (5668)$$

$$\tau_{\gamma,\delta,w,i}^{11} = \sum_{\alpha \in B} \tau_{\gamma,\alpha}^{10} \tau_{\delta,\alpha,w}^7 \tau_{\gamma,\alpha,i}^9 \quad (3r_D r_T^2 r_V N_o) \quad (5656)$$

$$\tau_{\gamma,\delta,w}^9 = \sum_{i \in O} {}^2D_{i,w}^4 Y_{i,\gamma}^4 Y_{i,\delta}^{4,*} \quad (3r_D r_T^2 N_o) \quad (5669)$$

$$\tau_{\gamma,w,i}^{12} = \sum_{\delta \in A} \tau_{\delta,\gamma,w}^0 \tau_{\delta,\gamma,w,i}^{11} \quad (2r_D r_T^2 N_o) \quad (5657)$$

$$\tau_{\gamma,\delta,w}^{10} = \sum_{\epsilon \in A} Z_{\delta,\epsilon}^* \tau_{\gamma,\epsilon,w}^8 \tau_{\gamma,\epsilon,w}^9 \quad (3r_D r_T^3) \quad (5670)$$

$${}^2R_{i,\gamma}^2 \leftarrow \sum_{w \in D} \frac{1}{4} {}^2D_{i,w}^2 \tau_{\gamma,w,i}^{12} \quad (2r_D r_T N_o) \quad (5658)$$

$$\tau_{\gamma,\delta,w}^{11} = \sum_{\epsilon \in A} Z_{\gamma,\epsilon} \tau_{\epsilon,\delta,w}^{10} \quad (2r_D r_T^3) \quad (5671)$$

Raw expression

$${}^2R_{i,\epsilon}^2 \leftarrow \sum_{\gamma \in A} \sum_{j \in O} \sum_{k \in O} \sum_{l \in O} \sum_{a \in V} \sum_{b \in V} \sum_{c \in V} \sum_{d \in V} \frac{1}{4} Y_{a,\epsilon}^{1,*} Z_{\epsilon,\gamma}^* Y_{b,\gamma}^{3,*} Y_{j,\gamma}^{4,*} {}^2D_{a,i,b,j} {}^2T_{c,i,b,j} {}^2T_{d,k,a,l} V_{k,c,l,d} \quad (5659)$$

$${}^2R_{i,\gamma}^2 \leftarrow \sum_{\delta \in A} \sum_{w \in D} \frac{1}{4} {}^2D_{i,w}^2 Y_{i,\delta}^2 \tau_{\delta,\gamma,w}^{11} \tau_{\delta,\gamma,w}^7 \quad (4r_D r_T^2 N_o) \quad (5672)$$

Raw expression

$${}^2R_{i,\epsilon}^2 \leftarrow \sum_{\gamma \in A} \sum_{j \in O} \sum_{k \in O} \sum_{l \in O} \sum_{a \in V} \sum_{b \in V} \sum_{c \in V} \sum_{d \in V} \frac{1}{4} Y_{a,\epsilon}^{1,*} Z_{\epsilon,\gamma}^* Y_{b,\gamma}^{3,*} Y_{j,\gamma}^{4,*} {}^2D_{a,i,b,j} {}^2T_{c,i,b,k} {}^2T_{d,j,a,l} V_{l,c,k,d} \quad (5673)$$

Factorized expression

$$\tau_{\gamma,\alpha}^0 = \sum_{a \in V} W_{a,\alpha}^4 Y_{a,\gamma}^1 \quad (2r_T r_V N_v) \quad (5660)$$

Factorized expression

$$\tau_{\gamma,\alpha,i}^1 = \sum_{\beta \in B} X_{\alpha,\beta} W_{i,\beta}^3 \tau_{\gamma,\beta}^0 \quad (3r_T r_V^2 N_o) \quad (5661)$$

$$\tau_{\gamma,\delta,w}^0 = \sum_{a \in V} {}^2D_{a,w}^1 Y_{a,\gamma}^3 Y_{a,\delta}^{1,*} \quad (3r_D r_T^2 N_v) \quad (5674)$$

$$\tau_{\gamma,\alpha}^2 = \sum_{i \in O} W_{i,\alpha}^1 Y_{i,\gamma}^2 \quad (2r_T r_V N_o) \quad (5662)$$

$$\tau_{\gamma,\delta,w}^1 = \sum_{a \in V} {}^2D_{a,w}^3 Y_{a,\gamma}^3 Y_{a,\delta}^{3,*} \quad (3r_D r_T^2 N_v) \quad (5675)$$

$$\tau_{\gamma,\alpha}^3 = \sum_{\delta \in A} \sum_{i \in O} Z_{\delta,\gamma} Y_{i,\gamma}^4 \tau_{\delta,\alpha}^2 \tau_{\delta,\alpha,i}^1 \quad (4r_T^2 r_V N_o) \quad (5663)$$

$$\tau_{\gamma,\alpha}^2 = \sum_{a \in V} W_{a,\alpha}^4 Y_{a,\gamma}^1 \quad (2r_T r_V N_v) \quad (5676)$$

$$\tau_{\gamma,a}^4 = \sum_{\alpha \in B} W_{a,\alpha}^2 \tau_{\gamma,\alpha}^3 \quad (2r_T r_V N_v) \quad (5664)$$

$$\tau_{\gamma,\alpha,i}^3 = \sum_{\beta \in B} X_{\alpha,\beta} W_{i,\beta}^3 \tau_{\gamma,\beta}^2 \quad (3r_T r_V^2 N_o) \quad (5677)$$

$$\tau_{a,b}^5 = \sum_{\gamma \in A} Y_{b,\gamma}^3 \tau_{\gamma,a}^4 \quad (2r_T N_v^2) \quad (5665)$$

$$\tau_{\gamma,\alpha}^4 = \sum_{i \in O} W_{i,\alpha}^1 Y_{i,\gamma}^2 \quad (2r_T r_V N_o) \quad (5678)$$

$$\tau_{\gamma,a}^6 = \sum_{b \in V} Y_{b,\gamma}^1 \tau_{b,a}^5 \quad (2r_T N_v^2) \quad (5666)$$

$$\tau_{\gamma,\alpha}^5 = \sum_{a \in V} W_{a,\alpha}^2 Y_{a,\gamma}^1 \quad (2r_T r_V N_v) \quad (5679)$$

$$\tau_{\gamma,\delta,i}^6 = \sum_{\alpha \in B} \tau_{\gamma,\alpha}^4 \tau_{\delta,\alpha}^5 \tau_{\gamma,\alpha,i}^3 \quad (3r_T^2 r_V N_o) \quad (5680)$$

$$\tau_{\gamma,\alpha}^5 = \sum_{\delta \in A} \sum_{i \in O} Z_{\delta,\gamma} Y_{i,\gamma}^4 \tau_{\delta,\alpha}^4 \tau_{\delta,\alpha,i}^3 \quad (4r_T^2 r_V N_o) \quad (5693)$$

$$\tau_{\gamma,\delta,\epsilon}^7 = \sum_{i \in O} Z_{\delta,\epsilon} Y_{i,\epsilon}^4 \tau_{\gamma,\delta,i}^6 \quad (3r_T^3 N_o) \quad (5681)$$

$$\tau_{\gamma,a}^6 = \sum_{\alpha \in B} W_{a,\alpha}^2 \tau_{\gamma,\alpha}^5 \quad (2r_T r_V N_v) \quad (5694)$$

$$\tau_{\gamma,\delta,i}^8 = \sum_{\epsilon \in A} Y_{i,\epsilon}^2 \tau_{\gamma,\epsilon,\delta}^7 \quad (2r_T^3 N_o) \quad (5682)$$

$$\tau_{a,b}^7 = \sum_{\gamma \in A} Y_{b,\gamma}^3 \tau_{\gamma,a}^6 \quad (2r_T N_v^2) \quad (5695)$$

$$\tau_{\gamma,\delta,w}^9 = \sum_{\epsilon \in A} \sum_{i \in O} {}^2D_{i,w}^4 Y_{i,\delta}^{4,*} \tau_{\epsilon,\delta,w}^1 \tau_{\gamma,\epsilon,i}^8 \quad (4r_D r_T^3 N_o) \quad (5683)$$

$$\tau_{\gamma,a}^8 = \sum_{b \in V} Y_{b,\gamma}^1 \tau_{b,a}^7 \quad (2r_T N_v^2) \quad (5696)$$

$$\tau_{\gamma,\delta,w}^{10} = \sum_{\epsilon \in A} Z_{\delta,\epsilon}^* \tau_{\gamma,\epsilon,w}^9 \quad (2r_D r_T^3) \quad (5684)$$

$$\tau_{\gamma,\delta,w}^9 = \sum_{a \in V} {}^2D_{a,w}^3 Y_{a,\delta}^{3,*} \tau_{\gamma,a}^8 \quad (3r_D r_T^2 N_v) \quad (5697)$$

$$\tau_{\gamma,\delta,w}^{11} = \sum_{\epsilon \in A} Z_{\epsilon,\gamma} \tau_{\epsilon,\delta,w}^{10} \quad (2r_D r_T^3) \quad (5685)$$

$$\tau_{\gamma,\delta,w}^{10} = \sum_{\epsilon \in A} Z_{\delta,\epsilon}^* \tau_{\gamma,\epsilon,w}^9 \quad (3r_D r_T^3) \quad (5698)$$

$${}^2R_{i,\gamma}^2 \leftarrow \sum_{\delta \in A} \sum_{w \in D} \frac{1}{4} {}^2D_{i,w}^2 Y_{i,\delta}^4 \tau_{\delta,\gamma,w}^0 \tau_{\delta,\gamma,w}^{11} \quad (4r_D r_T^2 N_o) \quad (5686)$$

$$\tau_{\gamma,\delta,w}^{11} = \sum_{\epsilon \in A} Z_{\epsilon,\gamma} \tau_{\epsilon,\delta,w}^{10} \quad (2r_D r_T^3) \quad (5699)$$

Raw expression

$${}^2R_{i,\epsilon}^2 \leftarrow \sum_{\gamma \in A} \sum_{j \in O} \sum_{k \in O} \sum_{l \in O} \sum_{a \in V} \sum_{b \in V} \sum_{c \in V} \sum_{d \in V} \frac{1}{4} Y_{a,\epsilon}^{1,*} Z_{\epsilon,\gamma}^* Y_{b,\gamma}^{3,*} Y_{j,\gamma}^{4,*} {}^2D_{a,i,b,j} {}^2T_{c,j,a,i} {}^2T_{d,k,b,l} V_{k,c,l,d} \quad (5687)$$

Factorized expression

$$\tau_{\gamma,\delta,w}^0 = \sum_{a \in V} {}^2D_{a,w}^1 Y_{a,\gamma}^3 Y_{a,\delta}^{1,*} \quad (3r_D r_T^2 N_v) \quad (5688)$$

$${}^2R_{i,\gamma}^2 \leftarrow \sum_{\delta \in A} \sum_{w \in D} \frac{1}{4} {}^2D_{i,w}^2 Y_{i,\delta}^4 \tau_{\delta,\gamma,w}^0 \tau_{\delta,\gamma,w}^{11} \quad (4r_D r_T^2 N_o) \quad (5700)$$

Raw expression

$${}^2R_{i,\epsilon}^2 \leftarrow \sum_{\gamma \in A} \sum_{j \in O} \sum_{k \in O} \sum_{l \in O} \sum_{a \in V} \sum_{b \in V} \sum_{c \in V} \sum_{d \in V} \frac{1}{4} Y_{a,\epsilon}^{1,*} Z_{\epsilon,\gamma}^* Y_{b,\gamma}^{3,*} Y_{j,\gamma}^{4,*} {}^2D_{a,i,b,j} {}^2T_{c,k,a,i} {}^2T_{d,j,b,l} V_{k,d,l,c} \quad (5701)$$

Factorized expression

$$\tau_{\gamma,\delta,w}^1 = \sum_{i \in O} {}^2D_{i,w}^4 Y_{i,\gamma}^2 Y_{i,\delta}^{4,*} \quad (3r_D r_T^2 N_o) \quad (5689)$$

$$\tau_{\gamma,\delta,w}^0 = \sum_{a \in V} {}^2D_{a,w}^1 Y_{a,\gamma}^3 Y_{a,\delta}^{1,*} \quad (3r_D r_T^2 N_v) \quad (5702)$$

$$\tau_{\gamma,\alpha}^2 = \sum_{a \in V} W_{a,\alpha}^4 Y_{a,\gamma}^1 \quad (2r_T r_V N_v) \quad (5690)$$

$$\tau_{\gamma,\alpha}^1 = \sum_{a \in V} W_{a,\alpha}^2 Y_{a,\gamma}^1 \quad (2r_T r_V N_v) \quad (5703)$$

$$\tau_{\gamma,\alpha,i}^3 = \sum_{\beta \in B} X_{\alpha,\beta} W_{i,\beta}^3 \tau_{\gamma,\beta}^2 \quad (3r_T r_V^2 N_o) \quad (5691)$$

$$\tau_{\gamma,\alpha,i}^2 = \sum_{\beta \in B} W_{i,\beta}^1 X_{\beta,\alpha} \tau_{\gamma,\beta}^1 \quad (3r_T r_V^2 N_o) \quad (5704)$$

$$\tau_{\gamma,\alpha}^4 = \sum_{i \in O} W_{i,\alpha}^1 Y_{i,\gamma}^2 \quad (2r_T r_V N_o) \quad (5692)$$

$$\tau_{\gamma,\alpha}^3 = \sum_{i \in O} W_{i,\alpha}^3 Y_{i,\gamma}^2 \quad (2r_T r_V N_o) \quad (5705)$$

### A. Contributions from $H$

$$\tau_{\gamma,\alpha}^4 = \sum_{a \in V} W_{a,\alpha}^4 Y_{a,\gamma}^1 \quad (2r_T r_V N_v) \quad (5706)$$

$$\tau_{\gamma,\delta,i}^5 = \sum_{\alpha \in B} \tau_{\gamma,\alpha}^3 \tau_{\delta,\alpha}^4 \tau_{\gamma,\alpha,i}^2 \quad (3r_T^2 r_V N_o) \quad (5707)$$

$$\tau_{\gamma,\delta,\epsilon}^6 = \sum_{i \in O} Z_{\delta,\epsilon} Y_{i,\epsilon}^4 \tau_{\gamma,\delta,i}^5 \quad (3r_T^3 N_o) \quad (5708)$$

$$\tau_{\gamma,\delta,i}^7 = \sum_{\epsilon \in A} Y_{i,\epsilon}^2 \tau_{\gamma,\epsilon,\delta}^6 \quad (2r_T^3 N_o) \quad (5709)$$

$$\tau_{\gamma,\delta,w}^8 = \sum_{a \in V} {}^2D_{a,w}^3 Y_{a,\gamma}^3 Y_{a,\delta}^{3,*} \quad (3r_D r_T^2 N_v) \quad (5710)$$

$$\tau_{\gamma,\delta,w}^9 = \sum_{i \in O} {}^2D_{i,w}^4 Y_{i,\gamma}^4 Y_{i,\delta}^{4,*} \quad (3r_D r_T^2 N_o) \quad (5711)$$

$$\tau_{\gamma,\delta,w}^{10} = \sum_{\epsilon \in A} Z_{\delta,\epsilon}^* \tau_{\gamma,\epsilon,w}^8 \tau_{\gamma,\epsilon,w}^9 \quad (3r_D r_T^3) \quad (5712)$$

$$\tau_{\gamma,\delta,w}^{11} = \sum_{\epsilon \in A} Z_{\gamma,\epsilon} \tau_{\epsilon,\delta,w}^{10} \quad (2r_D r_T^3) \quad (5713)$$

$$\tau_{\gamma,\delta,w,i}^{12} = \sum_{\epsilon \in A} \tau_{\epsilon,\delta,w}^{11} \tau_{\epsilon,\gamma,i}^7 \quad (2r_D r_T^3 N_o) \quad (5714)$$

$$\tau_{\gamma,w,i}^{13} = \sum_{\delta \in A} \tau_{\delta,\gamma,w}^0 \tau_{\delta,\gamma,w,i}^{12} \quad (2r_D r_T^2 N_o) \quad (5715)$$

$${}^2R_{i,\gamma}^2 \leftarrow \sum_{w \in D} \frac{1}{4} {}^2D_{i,w}^2 \tau_{\gamma,w,i}^{13} \quad (2r_D r_T N_o) \quad (5716)$$

## IX. THC-RCCSD DOUBLES ( $Z$ FACTOR) EQUATION

Here expressions for a THC-RCCSD doubles residual, projected against all factors except  $Z$ , are given along with their cost

Raw expression

$${}^2R_{\epsilon,\zeta}^z \leftarrow \sum_{i \in O} \sum_{j \in O} \sum_{a \in V} \sum_{b \in V} Y_{a,\epsilon}^{1,*} Y_{i,\epsilon}^{2,*} Y_{b,\zeta}^{3,*} Y_{j,\zeta}^{4,*} {}^2D_{a,i,b,j}^{a,i,b,j} V_{a,i,b,j} \quad (5717)$$

Factorized expression

$$\tau_{\gamma,\alpha,w}^0 = \sum_{a \in V} {}^2D_{a,w}^3 W_{a,\alpha}^3 Y_{a,\gamma}^{3,*} \quad (3r_D r_T r_V N_v) \quad (5718)$$

$$\tau_{\gamma,\alpha,w}^1 = \sum_{i \in O} {}^2D_{i,w}^4 W_{i,\alpha}^4 Y_{i,\gamma}^{4,*} \quad (3r_D r_T r_V N_o) \quad (5719)$$

$$\tau_{\gamma,\alpha,w}^2 = \sum_{\beta \in B} X_{\alpha,\beta} \tau_{\gamma,\beta,w}^0 \tau_{\gamma,\beta,w}^1 \quad (3r_D r_T r_V^2) \quad (5720)$$

$$\tau_{\gamma,\alpha,w}^3 = \sum_{a \in V} {}^2D_{a,w}^1 W_{a,\alpha}^1 Y_{a,\gamma}^{1,*} \quad (3r_D r_T r_V N_v) \quad (5721)$$

$$\tau_{\gamma,\alpha,w}^4 = \sum_{i \in O} {}^2D_{i,w}^2 W_{i,\alpha}^2 Y_{i,\gamma}^{2,*} \quad (3r_D r_T r_V N_o) \quad (5722)$$

$${}^2R_{\gamma,\delta}^z \leftarrow \sum_{\alpha \in B} \sum_{w \in D} \tau_{\delta,\alpha,w}^2 \tau_{\gamma,\alpha,w}^3 \tau_{\gamma,\alpha,w}^4 \quad (3r_D r_T^2 r_V) \quad (5723)$$

### B. Contributions from $(H^1 T)_c$

Raw expression

$${}^2R_{\epsilon,\zeta}^z \leftarrow - \sum_{i \in O} \sum_{j \in O} \sum_{k \in O} \sum_{a \in V} \sum_{b \in V} {}^1T_{a,k} Y_{a,\epsilon}^{1,*} Y_{i,\epsilon}^{2,*} Y_{b,\zeta}^{3,*} Y_{j,\zeta}^{4,*} {}^2D_{a,i,b,j}^{a,i,b,j} V_{b,j,k,i} \quad (5724)$$

Factorized expression

$$\tau_{\gamma,w,i}^0 = \sum_{a \in V} {}^2D_{a,w}^1 {}^1T_{a,i} Y_{a,\gamma}^{1,*} \quad (3r_D r_T N_o N_v) \quad (5725)$$

$$\tau_{\gamma,\alpha,w}^1 = \sum_{i \in O} W_{i,\alpha}^3 \tau_{\gamma,w,i}^0 \quad (2r_D r_T r_V N_o) \quad (5726)$$



$$\tau_{\gamma,\alpha,w}^2 = \sum_{i \in O} {}^2D_{i,w}^2 W_{i,\alpha}^4 Y_{i,\gamma}^{2,*} \quad (3r_D r_T r_V N_o) \quad (5727)$$

$$\tau_{\gamma,\alpha,w}^3 = \sum_{a \in V} {}^2D_{a,w}^3 W_{a,\alpha}^1 Y_{a,\gamma}^{3,*} \quad (3r_D r_T r_V N_v) \quad (5728)$$

$$\tau_{\gamma,\alpha,w}^4 = \sum_{i \in O} {}^2D_{i,w}^4 W_{i,\alpha}^2 Y_{i,\gamma}^{4,*} \quad (3r_D r_T r_V N_o) \quad (5729)$$

$$\tau_{\gamma,\alpha,w}^5 = \sum_{\beta \in B} X_{\beta,\alpha} \tau_{\gamma,\beta,w}^3 \tau_{\gamma,\beta,w}^4 \quad (3r_D r_T r_V^2) \quad (5730)$$

$${}^2R_{\gamma,\delta}^z \leftarrow - \sum_{\alpha \in B} \sum_{w \in D} \tau_{\gamma,\alpha,w}^1 \tau_{\gamma,\alpha,w}^2 \tau_{\delta,\alpha,w}^5 \quad (3r_D r_T^2 r_V) \quad (5731)$$

Raw expression

$${}^2R_{\epsilon,\zeta}^z \leftarrow - \sum_{i \in O} \sum_{j \in O} \sum_{k \in O} \sum_{a \in V} \sum_{b \in V} {}^1T_{b,k} Y_{a,\epsilon}^{1,*} Y_{i,\epsilon}^{2,*} Y_{b,\zeta}^{3,*} Y_{j,\zeta}^{4,*} {}^2D_{a,i,b,j} V_{a,i,k,j} \quad (5732)$$

Factorized expression

$$\tau_{\gamma,w,i}^0 = \sum_{a \in V} {}^2D_{a,w}^3 {}^1T_{a,i} Y_{a,\gamma}^{3,*} \quad (3r_D r_T N_o N_v) \quad (5733)$$

$$\tau_{\gamma,\alpha,w}^1 = \sum_{i \in O} W_{i,\alpha}^3 \tau_{\gamma,w,i}^0 \quad (2r_D r_T r_V N_o) \quad (5734)$$

$$\tau_{\gamma,\alpha,w}^2 = \sum_{i \in O} {}^2D_{i,w}^4 W_{i,\alpha}^4 Y_{i,\gamma}^{4,*} \quad (3r_D r_T r_V N_o) \quad (5735)$$

$$\tau_{\gamma,\alpha,w}^3 = \sum_{a \in V} {}^2D_{a,w}^1 W_{a,\alpha}^1 Y_{a,\gamma}^{1,*} \quad (3r_D r_T r_V N_v) \quad (5736)$$

$$\tau_{\gamma,\alpha,w}^4 = \sum_{i \in O} {}^2D_{i,w}^2 W_{i,\alpha}^2 Y_{i,\gamma}^{2,*} \quad (3r_D r_T r_V N_o) \quad (5737)$$

$$\tau_{\gamma,\alpha,w}^5 = \sum_{\beta \in B} X_{\beta,\alpha} \tau_{\gamma,\beta,w}^3 \tau_{\gamma,\beta,w}^4 \quad (3r_D r_T r_V^2) \quad (5738)$$

$${}^2R_{\gamma,\delta}^z \leftarrow - \sum_{\alpha \in B} \sum_{w \in D} \tau_{\delta,\alpha,w}^1 \tau_{\delta,\alpha,w}^2 \tau_{\gamma,\alpha,w}^5 \quad (3r_D r_T^2 r_V) \quad (5739)$$

Raw expression

$${}^2R_{\epsilon,\zeta}^z \leftarrow \sum_{i \in O} \sum_{j \in O} \sum_{a \in V} \sum_{b \in V} \sum_{c \in V} {}^1T_{c,i} Y_{a,\epsilon}^{1,*} Y_{i,\epsilon}^{2,*} Y_{b,\zeta}^{3,*} Y_{j,\zeta}^{4,*} {}^2D_{a,i,b,j} V_{a,c,b,j} \quad (5740)$$

Factorized expression

$$\tau_{\gamma,\alpha,w}^0 = \sum_{a \in V} {}^2D_{a,w}^3 W_{a,\alpha}^3 Y_{a,\gamma}^{3,*} \quad (3r_D r_T r_V N_v) \quad (5741)$$

$$\tau_{\gamma,\alpha,w}^1 = \sum_{i \in O} {}^2D_{i,w}^4 W_{i,\alpha}^4 Y_{i,\gamma}^{4,*} \quad (3r_D r_T r_V N_o) \quad (5742)$$

$$\tau_{\gamma,\alpha,w}^2 = \sum_{\beta \in B} X_{\alpha,\beta} \tau_{\gamma,\beta,w}^0 \tau_{\gamma,\beta,w}^1 \quad (3r_D r_T r_V^2) \quad (5743)$$

$$\tau_{\alpha,i}^3 = \sum_{a \in V} {}^1T_{a,i} W_{a,\alpha}^2 \quad (2r_V N_o N_v) \quad (5744)$$

$$\tau_{\gamma,\alpha,w}^4 = \sum_{i \in O} {}^2D_{i,w}^2 Y_{i,\gamma}^{2,*} \tau_{\alpha,i}^3 \quad (3r_D r_T r_V N_o) \quad (5745)$$

$$\tau_{\gamma,\alpha,w}^5 = \sum_{a \in V} {}^2D_{a,w}^1 W_{a,\alpha}^1 Y_{a,\gamma}^{1,*} \quad (3r_D r_T r_V N_v) \quad (5746)$$

$${}^2R_{\gamma,\delta}^z \leftarrow \sum_{\alpha \in B} \sum_{w \in D} \tau_{\delta,\alpha,w}^2 \tau_{\gamma,\alpha,w}^4 \tau_{\gamma,\alpha,w}^5 \quad (3r_D r_T^2 r_V) \quad (5747)$$

Raw expression

$${}^2R_{\epsilon,\zeta}^z \leftarrow \sum_{i \in O} \sum_{j \in O} \sum_{a \in V} \sum_{b \in V} \sum_{c \in V} {}^1T_{c,j} Y_{a,\epsilon}^{1,*} Y_{i,\epsilon}^{2,*} Y_{b,\zeta}^{3,*} Y_{j,\zeta}^{4,*} {}^2D_{a,i,b,j} V_{a,i,b,c} \quad (5748)$$

Factorized expression

$$\tau_{\alpha,i}^0 = \sum_{a \in V} {}^1T_{a,i} W_{a,\alpha}^4 \quad (2r_V N_o N_v) \quad (5749)$$

$$\tau^1_{\gamma,\alpha,w} = \sum_{i \in O} {}^2D^4_{i,w} Y^{4,*}_{i,\gamma} \tau^0_{\alpha,i} \quad (3r_D r_T r_V N_o) \quad (5750)$$

$$\tau^4_{\gamma,\alpha,w} = \sum_{i \in O} {}^2D^2_{i,w} Y^{2,*}_{i,\gamma} \tau^3_{\alpha,i} \quad (3r_D r_T r_V N_o) \quad (5761)$$

$$\tau^2_{\gamma,\alpha,w} = \sum_{a \in V} {}^2D^3_{a,w} W^3_{a,\alpha} Y^{3,*}_{a,\gamma} \quad (3r_D r_T r_V N_v) \quad (5751)$$

$$\tau^5_{\gamma,w,i} = \sum_{a \in V} {}^2D^1_{a,w} {}^1T_{a,i} Y^{1,*}_{a,\gamma} \quad (3r_D r_T N_o N_v) \quad (5762)$$

$$\tau^3_{\gamma,\alpha,w} = \sum_{\beta \in B} X_{\alpha,\beta} \tau^1_{\gamma,\beta,w} \tau^2_{\gamma,\beta,w} \quad (3r_D r_T r_V^2) \quad (5752)$$

$$\tau^6_{\gamma,\alpha,w} = \sum_{i \in O} W^3_{i,\alpha} \tau^5_{\gamma,w,i} \quad (2r_D r_T r_V N_o) \quad (5763)$$

$$\tau^4_{\gamma,\alpha,w} = \sum_{a \in V} {}^2D^1_{a,w} W^1_{a,\alpha} Y^{1,*}_{a,\gamma} \quad (3r_D r_T r_V N_v) \quad (5753)$$

$${}^2R^z_{\gamma,\delta} \leftarrow - \sum_{\alpha \in B} \sum_{w \in D} \tau^2_{\delta,\alpha,w} \tau^4_{\gamma,\alpha,w} \tau^6_{\gamma,\alpha,w} \quad (3r_D r_T^2 r_V) \quad (5764)$$

$$\tau^5_{\gamma,\alpha,w} = \sum_{i \in O} {}^2D^2_{i,w} W^2_{i,\alpha} Y^{2,*}_{i,\gamma} \quad (3r_D r_T r_V N_o) \quad (5754)$$

Raw expression

$${}^2R^z_{\epsilon,\zeta} \leftarrow - \sum_{i \in O} \sum_{j \in O} \sum_{k \in O} \sum_{a \in V} \sum_{b \in V} \sum_{c \in V} {}^1T_{a,k} {}^1T_{c,j} Y^{1,*}_{a,\epsilon} Y^{2,*}_{i,\epsilon} Y^{3,*}_{b,\zeta} Y^{4,*}_{j,\zeta} {}^2D^{a,i,b,j}_{b,c,k,i} \quad (5765)$$

$${}^2R^z_{\gamma,\delta} \leftarrow \sum_{\alpha \in B} \sum_{w \in D} \tau^3_{\delta,\alpha,w} \tau^4_{\gamma,\alpha,w} \tau^5_{\gamma,\alpha,w} \quad (3r_D r_T^2 r_V) \quad (5755)$$

Factorized expression

$$\tau^0_{\alpha,i} = \sum_{a \in V} {}^1T_{a,i} W^2_{a,\alpha} \quad (2r_V N_o N_v) \quad (5766)$$

### C. Contributions from $(H^1 T^1 T)_c$

Raw expression

$${}^2R^z_{\epsilon,\zeta} \leftarrow - \sum_{i \in O} \sum_{j \in O} \sum_{k \in O} \sum_{a \in V} \sum_{b \in V} \sum_{c \in V} {}^1T_{a,k} {}^1T_{c,i} Y^{1,*}_{a,\epsilon} Y^{2,*}_{i,\epsilon} Y^{3,*}_{b,\zeta} Y^{4,*}_{j,\zeta} {}^2D^{a,i,b,j}_{b,j,k,c} \quad (5756)$$

Factorized expression

$$\tau^0_{\gamma,\alpha,w} = \sum_{a \in V} {}^2D^3_{a,w} W^1_{a,\alpha} Y^{3,*}_{a,\gamma} \quad (3r_D r_T r_V N_v) \quad (5757)$$

$$\tau^1_{\gamma,\alpha,w} = \sum_{i \in O} {}^2D^4_{i,w} Y^{4,*}_{i,\gamma} \tau^0_{\alpha,i} \quad (3r_D r_T r_V N_o) \quad (5767)$$

$$\tau^2_{\gamma,\alpha,w} = \sum_{a \in V} {}^2D^3_{a,w} W^1_{a,\alpha} Y^{3,*}_{a,\gamma} \quad (3r_D r_T r_V N_v) \quad (5768)$$

$$\tau^1_{\gamma,\alpha,w} = \sum_{i \in O} {}^2D^4_{i,w} W^2_{i,\alpha} Y^{4,*}_{i,\gamma} \quad (3r_D r_T r_V N_o) \quad (5758)$$

$$\tau^4_{\gamma,w,i} = \sum_{a \in V} {}^2D^1_{a,w} {}^1T_{a,i} Y^{1,*}_{a,\gamma} \quad (3r_D r_T N_o N_v) \quad (5770)$$

$$\tau^2_{\gamma,\alpha,w} = \sum_{\beta \in B} X_{\beta,\alpha} \tau^0_{\gamma,\beta,w} \tau^1_{\gamma,\beta,w} \quad (3r_D r_T r_V^2) \quad (5759)$$

$$\tau^5_{\gamma,\alpha,w} = \sum_{i \in O} W^3_{i,\alpha} \tau^4_{\gamma,w,i} \quad (2r_D r_T r_V N_o) \quad (5771)$$

$$\tau^3_{\alpha,i} = \sum_{a \in V} {}^1T_{a,i} W^4_{a,\alpha} \quad (2r_V N_o N_v) \quad (5760)$$

$$\tau^6_{\gamma,\alpha,w} = \sum_{i \in O} {}^2D^2_{i,w} W^4_{i,\alpha} Y^{2,*}_{i,\gamma} \quad (3r_D r_T r_V N_o) \quad (5772)$$

$${}^2R^z_{\gamma,\delta} \leftarrow - \sum_{\alpha \in B} \sum_{w \in D} \tau^3_{\delta,\alpha,w} \tau^5_{\gamma,\alpha,w} \tau^6_{\gamma,\alpha,w} \quad (3r_D r_T^2 r_V) \quad (5773)$$

Raw expression

$${}^2R^z_{\epsilon,\zeta} \leftarrow - \sum_{i \in O} \sum_{j \in O} \sum_{k \in O} \sum_{a \in V} \sum_{b \in V} \sum_{c \in V} {}^1T_{b,k} {}^1T_{c,i} Y^{1,*}_{a,\epsilon} Y^{2,*}_{i,\epsilon} Y^{3,*}_{b,\zeta} Y^{4,*}_{j,\zeta} {}^2D^{a,i,b,j} V_{a,c,k,j} \quad (5774)$$

Factorized expression

$$\tau^0_{\gamma,w,i} = \sum_{a \in V} {}^2D^3_{a,w} {}^1T_{a,i} Y^{3,*}_{a,\gamma} \quad (3r_D r_T N_o N_v) \quad (5775)$$

$$\tau^1_{\gamma,\alpha,w} = \sum_{i \in O} W^3_{i,\alpha} \tau^0_{\gamma,w,i} \quad (2r_D r_T r_V N_o) \quad (5776)$$

$$\tau^2_{\gamma,\alpha,w} = \sum_{i \in O} {}^2D^4_{i,w} W^4_{i,\alpha} Y^{4,*}_{i,\gamma} \quad (3r_D r_T r_V N_o) \quad (5777)$$

$$\tau^3_{\alpha,i} = \sum_{a \in V} {}^1T_{a,i} W^2_{a,\alpha} \quad (2r_V N_o N_v) \quad (5778)$$

$$\tau^4_{\gamma,\alpha,w} = \sum_{i \in O} {}^2D^2_{i,w} Y^{2,*}_{i,\gamma} \tau^3_{\alpha,i} \quad (3r_D r_T r_V N_o) \quad (5779)$$

$$\tau^5_{\gamma,\alpha,w} = \sum_{a \in V} {}^2D^1_{a,w} W^1_{a,\alpha} Y^{1,*}_{a,\gamma} \quad (3r_D r_T r_V N_v) \quad (5780)$$

$$\tau^6_{\gamma,\alpha,w} = \sum_{\beta \in B} X_{\beta,\alpha} \tau^4_{\gamma,\beta,w} \tau^5_{\gamma,\beta,w} \quad (3r_D r_T r_V^2) \quad (5781)$$

$${}^2R^z_{\gamma,\delta} \leftarrow - \sum_{\alpha \in B} \sum_{w \in D} \tau^1_{\delta,\alpha,w} \tau^2_{\delta,\alpha,w} \tau^6_{\gamma,\alpha,w} \quad (3r_D r_T^2 r_V) \quad (5782)$$

Raw expression

$${}^2R^z_{\epsilon,\zeta} \leftarrow - \sum_{i \in O} \sum_{j \in O} \sum_{k \in O} \sum_{a \in V} \sum_{b \in V} \sum_{c \in V} {}^1T_{b,k} {}^1T_{c,j} Y^{1,*}_{a,\epsilon} Y^{2,*}_{i,\epsilon} Y^{3,*}_{b,\zeta} Y^{4,*}_{j,\zeta} {}^2D^{a,i,b,j} V_{a,i,k,c} \quad (5783)$$

Factorized expression

$$\tau^0_{\alpha,i} = \sum_{a \in V} {}^1T_{a,i} W^4_{a,\alpha} \quad (2r_V N_o N_v) \quad (5784)$$

$$\tau^1_{\gamma,\alpha,w} = \sum_{i \in O} {}^2D^4_{i,w} Y^{4,*}_{i,\gamma} \tau^0_{\alpha,i} \quad (3r_D r_T r_V N_o) \quad (5785)$$

$$\tau^2_{\gamma,w,i} = \sum_{a \in V} {}^2D^3_{a,w} {}^1T_{a,i} Y^{3,*}_{a,\gamma} \quad (3r_D r_T N_o N_v) \quad (5786)$$

$$\tau^3_{\gamma,\alpha,w} = \sum_{i \in O} W^3_{i,\alpha} \tau^2_{\gamma,w,i} \quad (2r_D r_T r_V N_o) \quad (5787)$$

$$\tau^4_{\gamma,\alpha,w} = \sum_{a \in V} {}^2D^1_{a,w} W^1_{a,\alpha} Y^{1,*}_{a,\gamma} \quad (3r_D r_T r_V N_v) \quad (5788)$$

$$\tau^5_{\gamma,\alpha,w} = \sum_{i \in O} {}^2D^2_{i,w} W^2_{i,\alpha} Y^{2,*}_{i,\gamma} \quad (3r_D r_T r_V N_o) \quad (5789)$$

$$\tau^6_{\gamma,\alpha,w} = \sum_{\beta \in B} X_{\beta,\alpha} \tau^4_{\gamma,\beta,w} \tau^5_{\gamma,\beta,w} \quad (3r_D r_T r_V^2) \quad (5790)$$

$${}^2R^z_{\gamma,\delta} \leftarrow - \sum_{\alpha \in B} \sum_{w \in D} \tau^1_{\delta,\alpha,w} \tau^3_{\delta,\alpha,w} \tau^6_{\gamma,\alpha,w} \quad (3r_D r_T^2 r_V) \quad (5791)$$

Raw expression

$${}^2R^z_{\epsilon,\zeta} \leftarrow \sum_{i \in O} \sum_{j \in O} \sum_{k \in O} \sum_{l \in O} \sum_{a \in V} \sum_{b \in V} {}^1T_{a,k} {}^1T_{b,l} Y^{1,*}_{a,\epsilon} Y^{2,*}_{i,\epsilon} Y^{3,*}_{b,\zeta} Y^{4,*}_{j,\zeta} {}^2D^{a,i,b,j} V_{k,i,l,j} \quad (5792)$$

Factorized expression

$$\tau^0_{\gamma,w,i} = \sum_{a \in V} {}^2D^3_{a,w} {}^1T_{a,i} Y^{3,*}_{a,\gamma} \quad (3r_D r_T N_o N_v) \quad (5793)$$

$$\tau^1_{\gamma,\alpha,w} = \sum_{i \in O} W^3_{i,\alpha} \tau^0_{\gamma,w,i} \quad (2r_D r_T r_V N_o) \quad (5794)$$

$$\tau^2_{\gamma,\alpha,w} = \sum_{i \in O} {}^2D^4_{i,w} W^4_{i,\alpha} Y^{4,*}_{i,\gamma} \quad (3r_D r_T r_V N_o) \quad (5795)$$

### D. Contributions from $(H^2T)_c$

$$\tau_{\gamma,w,i}^3 = \sum_{a \in V} {}^2D_{a,w}^1 {}^1T_{a,i} Y_{a,\gamma}^{1,*} \quad (3r_D r_T N_o N_v) \quad (5796)$$

$$\tau_{\gamma,\alpha,w}^4 = \sum_{i \in O} W_{i,\alpha}^1 \tau_{\gamma,w,i}^3 \quad (2r_D r_T r_V N_o) \quad (5797)$$

$$\tau_{\gamma,\alpha,w}^5 = \sum_{i \in O} {}^2D_{i,w}^2 W_{i,\alpha}^2 Y_{i,\gamma}^{2,*} \quad (3r_D r_T r_V N_o) \quad (5798)$$

$$\tau_{\gamma,\alpha,w}^6 = \sum_{\beta \in B} X_{\beta,\alpha} \tau_{\gamma,\beta,w}^4 \tau_{\gamma,\beta,w}^5 \quad (3r_D r_T r_V^2) \quad (5799)$$

$${}^2R_{\gamma,\delta}^z \leftarrow \sum_{\alpha \in B} \sum_{w \in D} \tau_{\delta,\alpha,w}^1 \tau_{\delta,\alpha,w}^2 \tau_{\gamma,\alpha,w}^6 \quad (3r_D r_T^2 r_V) \quad (5800)$$

Raw expression

$${}^2R_{\epsilon,\zeta}^z \leftarrow \sum_{i \in O} \sum_{j \in O} \sum_{a \in V} \sum_{b \in V} \sum_{c \in V} \sum_{d \in V} {}^1T_{c,i} {}^1T_{d,j} Y_{a,\epsilon}^{1,*} Y_{i,\epsilon}^{2,*} Y_{b,\zeta}^{3,*} Y_{j,\zeta}^{4,*} {}^2D_{a,i,b,j} V_{a,c,b,d} \quad (5801)$$

Factorized expression

$$\tau_{\alpha,i}^0 = \sum_{a \in V} {}^1T_{a,i} W_{a,\alpha}^4 \quad (2r_V N_o N_v) \quad (5802)$$

$$\tau_{\gamma,\alpha,w}^1 = \sum_{i \in O} {}^2D_{i,w}^4 Y_{i,\gamma}^{4,*} \tau_{\alpha,i}^0 \quad (3r_D r_T r_V N_o) \quad (5803)$$

$$\tau_{\gamma,\alpha,w}^2 = \sum_{a \in V} {}^2D_{a,w}^3 W_{a,\alpha}^3 Y_{a,\gamma}^{3,*} \quad (3r_D r_T r_V N_v) \quad (5804)$$

$$\tau_{\alpha,i}^3 = \sum_{a \in V} {}^1T_{a,i} W_{a,\alpha}^2 \quad (2r_V N_o N_v) \quad (5805)$$

$$\tau_{\gamma,\alpha,w}^4 = \sum_{i \in O} {}^2D_{i,w}^2 Y_{i,\gamma}^{2,*} \tau_{\alpha,i}^3 \quad (3r_D r_T r_V N_o) \quad (5806)$$

$$\tau_{\gamma,\alpha,w}^5 = \sum_{a \in V} {}^2D_{a,w}^1 W_{a,\alpha}^1 Y_{a,\gamma}^{1,*} \quad (3r_D r_T r_V N_v) \quad (5807)$$

$$\tau_{\gamma,\alpha,w}^6 = \sum_{\beta \in B} X_{\beta,\alpha} \tau_{\gamma,\beta,w}^4 \tau_{\gamma,\beta,w}^5 \quad (3r_D r_T r_V^2) \quad (5808)$$

$${}^2R_{\gamma,\delta}^z \leftarrow \sum_{\alpha \in B} \sum_{w \in D} \tau_{\delta,\alpha,w}^1 \tau_{\delta,\alpha,w}^2 \tau_{\gamma,\alpha,w}^6 \quad (3r_D r_T^2 r_V) \quad (5809)$$

Raw expression

$${}^2R_{\epsilon,\zeta}^z \leftarrow - \sum_{i \in O} \sum_{j \in O} \sum_{k \in O} \sum_{a \in V} \sum_{b \in V} \frac{1}{2} Y_{a,\epsilon}^{1,*} Y_{i,\epsilon}^{2,*} Y_{b,\zeta}^{3,*} Y_{j,\zeta}^{4,*} f_{k,i} {}^2D_{a,i,b,j} {}^2T_{a,k,b,j} \quad (5810)$$

Factorized expression

$$\tau_{\gamma,\delta,w}^0 = \sum_{i \in O} {}^2D_{i,w}^4 Y_{i,\gamma}^4 Y_{i,\delta}^{4,*} \quad (3r_D r_T^2 N_o) \quad (5811)$$

$$\tau_{\gamma,a}^1 = \sum_{b \in V} Y_{b,\gamma}^3 f_{a,b} \quad (2r_T N_v^2) \quad (5812)$$

$$\tau_{\gamma,\delta,w}^2 = \sum_{a \in V} {}^2D_{a,w}^3 Y_{a,\delta}^{3,*} \tau_{\gamma,a}^1 \quad (3r_D r_T^2 N_v) \quad (5813)$$

$$\tau_{\gamma,\delta,w}^3 = \sum_{a \in V} {}^2D_{a,w}^1 Y_{a,\gamma}^1 Y_{a,\delta}^{1,*} \quad (3r_D r_T^2 N_v) \quad (5814)$$

$$\tau_{\gamma,\delta,w}^4 = \sum_{i \in O} {}^2D_{i,w}^2 Y_{i,\gamma}^2 Y_{i,\delta}^{2,*} \quad (3r_D r_T^2 N_o) \quad (5815)$$

$$\tau_{\gamma,\delta,w}^5 = \sum_{\epsilon \in A} Z_{\epsilon,\gamma} \tau_{\epsilon,\delta,w}^3 \tau_{\epsilon,\delta,w}^4 \quad (3r_D r_T^3) \quad (5816)$$

$${}^2R_{\gamma,\delta}^z \leftarrow \sum_{\epsilon \in A} \sum_{w \in D} \frac{1}{2} \tau_{\epsilon,\delta,w}^0 \tau_{\epsilon,\delta,w}^2 \tau_{\epsilon,\gamma,w}^5 \quad (3r_D r_T^3) \quad (5817)$$

Raw expression

$${}^2R_{\epsilon,\zeta}^z \leftarrow - \sum_{i \in O} \sum_{j \in O} \sum_{k \in O} \sum_{a \in V} \sum_{b \in V} \frac{1}{2} Y_{a,\epsilon}^{1,*} Y_{i,\epsilon}^{2,*} Y_{b,\zeta}^{3,*} Y_{j,\zeta}^{4,*} f_{k,i} {}^2D_{a,i,b,j} {}^2T_{b,j,a,k} \quad (5818)$$

Factorized expression

$$\tau_{\gamma,\delta,w}^0 = \sum_{a \in V} {}^2D_{a,w}^3 Y_{a,\gamma}^1 Y_{a,\delta}^{3,*} \quad (3r_D r_T^2 N_v) \quad (5819)$$

$$\tau_{\gamma,\delta,w}^1 = \sum_{i \in O} {}^2D_{i,w}^4 Y_{i,\gamma}^2 Y_{i,\delta}^{4,*} \quad (3r_D r_T^2 N_o) \quad (5820)$$

$$\tau_{\gamma,\delta,w}^2 = \sum_{\epsilon \in A} Z_{\epsilon,\gamma} \tau_{\epsilon,\delta,w}^0 \tau_{\epsilon,\delta,w}^1 \quad (3r_D r_T^3) \quad (5821)$$

$$\tau^3_{\gamma,\delta,w} = \sum_{i \in O} {}^2D^2_{i,w} Y^4_{i,\gamma} Y^{2,*}_{i,\delta} \quad (3r_D r_T^2 N_o) \quad (5822)$$

$$\tau^4_{\gamma,a} = \sum_{b \in V} Y^3_{b,\gamma} f_{a,b} \quad (2r_T N_v^2) \quad (5823)$$

$$\tau^5_{\gamma,\delta,w} = \sum_{a \in V} {}^2D^1_{a,w} Y^{1,*}_{a,\delta} \tau^4_{\gamma,a} \quad (3r_D r_T^2 N_v) \quad (5824)$$

$${}^2R^z_{\gamma,\delta} \leftarrow \sum_{\epsilon \in A} \sum_{w \in D} \frac{1}{2} \tau^2_{\epsilon,\delta,w} \tau^3_{\epsilon,\gamma,w} \tau^5_{\epsilon,\gamma,w} \quad (3r_D r_T^3) \quad (5825)$$

Raw expression

$${}^2R^z_{\epsilon,\zeta} \leftarrow - \sum_{i \in O} \sum_{j \in O} \sum_{k \in O} \sum_{a \in V} \sum_{b \in V} \frac{1}{2} Y^{1,*}_{a,\epsilon} Y^{2,*}_{i,\epsilon} Y^{3,*}_{b,\zeta} Y^{4,*}_{j,\zeta} f_{k,j} {}^2D^{a,i,b,j} {}^2T_{a,i,b,k} \quad (5826)$$

Factorized expression

$$\tau^0_{\gamma,\delta,w} = \sum_{a \in V} {}^2D^3_{a,w} Y^3_{a,\gamma} Y^{3,*}_{a,\delta} \quad (3r_D r_T^2 N_v) \quad (5827)$$

$$\tau^1_{\gamma,\delta,w} = \sum_{i \in O} {}^2D^4_{i,w} Y^4_{i,\gamma} Y^{4,*}_{i,\delta} \quad (3r_D r_T^2 N_o) \quad (5828)$$

$$\tau^2_{\gamma,\delta,w} = \sum_{i \in O} {}^2D^2_{i,w} Y^2_{i,\gamma} Y^{2,*}_{i,\delta} \quad (3r_D r_T^2 N_o) \quad (5829)$$

$$\tau^3_{\gamma,a} = \sum_{b \in V} Y^1_{b,\gamma} f_{a,b} \quad (2r_T N_v^2) \quad (5830)$$

$$\tau^4_{\gamma,\delta,w} = \sum_{a \in V} {}^2D^1_{a,w} Y^{1,*}_{a,\delta} \tau^3_{\gamma,a} \quad (3r_D r_T^2 N_v) \quad (5831)$$

$$\tau^5_{\gamma,\delta,w} = \sum_{\epsilon \in A} Z_{\epsilon,\gamma} \tau^2_{\epsilon,\delta,w} \tau^4_{\epsilon,\delta,w} \quad (3r_D r_T^3) \quad (5832)$$

$${}^2R^z_{\gamma,\delta} \leftarrow \sum_{\epsilon \in A} \sum_{w \in D} \frac{1}{2} \tau^0_{\epsilon,\delta,w} \tau^1_{\epsilon,\delta,w} \tau^5_{\epsilon,\gamma,w} \quad (3r_D r_T^3) \quad (5833)$$

Raw expression

$${}^2R^z_{\epsilon,\zeta} \leftarrow - \sum_{i \in O} \sum_{j \in O} \sum_{k \in O} \sum_{a \in V} \sum_{b \in V} \frac{1}{2} Y^{1,*}_{a,\epsilon} Y^{2,*}_{i,\epsilon} Y^{3,*}_{b,\zeta} Y^{4,*}_{j,\zeta} f_{k,j} {}^2D^{a,i,b,j} {}^2T_{b,k,a,i} \quad (5834)$$

Factorized expression

$$\tau^0_{\gamma,\delta,w} = \sum_{i \in O} {}^2D^4_{i,w} Y^2_{i,\gamma} Y^{4,*}_{i,\delta} \quad (3r_D r_T^2 N_o) \quad (5835)$$

$$\tau^1_{\gamma,a} = \sum_{b \in V} Y^1_{b,\gamma} f_{a,b} \quad (2r_T N_v^2) \quad (5836)$$

$$\tau^2_{\gamma,\delta,w} = \sum_{a \in V} {}^2D^3_{a,w} Y^{3,*}_{a,\delta} \tau^1_{\gamma,a} \quad (3r_D r_T^2 N_v) \quad (5837)$$

$$\tau^3_{\gamma,\delta,w} = \sum_{\epsilon \in A} Z_{\epsilon,\gamma} \tau^0_{\epsilon,\delta,w} \tau^2_{\epsilon,\delta,w} \quad (3r_D r_T^3) \quad (5838)$$

$$\tau^4_{\gamma,\delta,w} = \sum_{a \in V} {}^2D^1_{a,w} Y^3_{a,\gamma} Y^{1,*}_{a,\delta} \quad (3r_D r_T^2 N_v) \quad (5839)$$

$$\tau^5_{\gamma,\delta,w} = \sum_{i \in O} {}^2D^2_{i,w} Y^4_{i,\gamma} Y^{2,*}_{i,\delta} \quad (3r_D r_T^2 N_o) \quad (5840)$$

$${}^2R^z_{\gamma,\delta} \leftarrow \sum_{\epsilon \in A} \sum_{w \in D} \frac{1}{2} \tau^3_{\epsilon,\delta,w} \tau^4_{\epsilon,\gamma,w} \tau^5_{\epsilon,\gamma,w} \quad (3r_D r_T^3) \quad (5841)$$

Raw expression

$${}^2R^z_{\epsilon,\zeta} \leftarrow \sum_{i \in O} \sum_{j \in O} \sum_{k \in O} \sum_{a \in V} \sum_{b \in V} \sum_{c \in V} Y^{1,*}_{a,\epsilon} Y^{2,*}_{i,\epsilon} Y^{3,*}_{b,\zeta} Y^{4,*}_{j,\zeta} {}^2D^{a,i,b,j} {}^2T_{a,i,c,k} V_{b,j,k,c} \quad (5842)$$

Factorized expression

$$\tau^0_{\gamma,\delta,w} = \sum_{a \in V} {}^2D^3_{a,w} Y^1_{a,\gamma} Y^{3,*}_{a,\delta} \quad (3r_D r_T^2 N_v) \quad (5843)$$

$$\tau^1_{\gamma,\delta,w} = \sum_{i \in O} {}^2D^4_{i,w} Y^2_{i,\gamma} Y^{4,*}_{i,\delta} \quad (3r_D r_T^2 N_o) \quad (5844)$$

$$\tau^2_{\gamma,\alpha,w} = \sum_{a \in V} {}^2D^1_{a,w} W^1_{a,\alpha} Y^{1,*}_{a,\gamma} \quad (3r_D r_T r_V N_v) \quad (5845)$$

$$\tau^3_{\gamma,\alpha,w} = \sum_{i \in O} {}^2D^2_{i,w} W^2_{i,\alpha} Y^{2,*}_{i,\gamma} \quad (3r_D r_T r_V N_o) \quad (5846)$$

$$\tau^4_{\gamma,\alpha} = \sum_{a \in V} W^4_{a,\alpha} Y^3_{a,\gamma} \quad (2r_T r_V N_v) \quad (5847)$$

$$\tau^5_{\gamma,\alpha} = \sum_{i \in O} W^3_{i,\alpha} Y^4_{i,\gamma} \quad (2r_T r_V N_o) \quad (5848)$$

$$\tau^6_{\gamma,\alpha} = \sum_{\beta \in B} X_{\alpha,\beta} \tau^4_{\gamma,\beta} \tau^5_{\gamma,\beta} \quad (3r_T r_V^2) \quad (5849)$$

$$\tau^7_{\gamma,\alpha} = \sum_{\delta \in A} Z_{\gamma,\delta} \tau^6_{\delta,\alpha} \quad (2r_T^2 r_V) \quad (5850)$$

$$\tau^8_{\gamma,\delta,w} = \sum_{\alpha \in B} \tau^7_{\gamma,\alpha} \tau^2_{\delta,\alpha,w} \tau^3_{\delta,\alpha,w} \quad (3r_D r_T^2 r_V) \quad (5851)$$

$${}^2R^z_{\gamma,\delta} \leftarrow \sum_{\epsilon \in A} \sum_{w \in D} \tau^0_{\epsilon,\delta,w} \tau^1_{\epsilon,\delta,w} \tau^8_{\epsilon,\gamma,w} \quad (3r_D r_T^3) \quad (5852)$$

Raw expression

$${}^2R^z_{\epsilon,\zeta} \leftarrow \sum_{i \in O} \sum_{j \in O} \sum_{k \in O} \sum_{a \in V} \sum_{b \in V} \sum_{c \in V} Y^{1,*}_{a,\epsilon} Y^{2,*}_{i,\epsilon} Y^{3,*}_{b,\zeta} Y^{4,*}_{j,\zeta} {}^2D^{a,i,b,j} {}^2T_{b,j,c,k} V_{a,i,k,c} \quad (5853)$$

Factorized expression

$$\tau^0_{\gamma,\delta,w} = \sum_{a \in V} {}^2D^3_{a,w} Y^3_{a,\gamma} Y^{3,*}_{a,\delta} \quad (3r_D r_T^2 N_v) \quad (5854)$$

$$\tau^1_{\gamma,\delta,w} = \sum_{i \in O} {}^2D^4_{i,w} Y^4_{i,\gamma} Y^{4,*}_{i,\delta} \quad (3r_D r_T^2 N_o) \quad (5855)$$

$$\tau^2_{\gamma,\alpha,w} = \sum_{a \in V} {}^2D^1_{a,w} W^1_{a,\alpha} Y^{1,*}_{a,\gamma} \quad (3r_D r_T r_V N_v) \quad (5856)$$

$$\tau^3_{\gamma,\alpha,w} = \sum_{i \in O} {}^2D^2_{i,w} W^2_{i,\alpha} Y^{2,*}_{i,\gamma} \quad (3r_D r_T r_V N_o) \quad (5857)$$

$$\tau^4_{\gamma,\alpha} = \sum_{a \in V} W^4_{a,\alpha} Y^1_{a,\gamma} \quad (2r_T r_V N_v) \quad (5858)$$

$$\tau^5_{\gamma,\alpha} = \sum_{i \in O} W^3_{i,\alpha} Y^2_{i,\gamma} \quad (2r_T r_V N_o) \quad (5859)$$

$$\tau^6_{\gamma,\alpha} = \sum_{\beta \in B} X_{\alpha,\beta} \tau^4_{\gamma,\beta} \tau^5_{\gamma,\beta} \quad (3r_T r_V^2) \quad (5860)$$

$$\tau^7_{\gamma,\alpha} = \sum_{\delta \in A} Z_{\delta,\gamma} \tau^6_{\delta,\alpha} \quad (2r_T^2 r_V) \quad (5861)$$

$$\tau^8_{\gamma,\delta,w} = \sum_{\alpha \in B} \tau^7_{\gamma,\alpha} \tau^2_{\delta,\alpha,w} \tau^3_{\delta,\alpha,w} \quad (3r_D r_T^2 r_V) \quad (5862)$$

$${}^2R^z_{\gamma,\delta} \leftarrow \sum_{\epsilon \in A} \sum_{w \in D} \tau^0_{\epsilon,\delta,w} \tau^1_{\epsilon,\delta,w} \tau^8_{\epsilon,\gamma,w} \quad (3r_D r_T^3) \quad (5863)$$

Raw expression

$${}^2R^z_{\epsilon,\zeta} \leftarrow \sum_{i \in O} \sum_{j \in O} \sum_{k \in O} \sum_{a \in V} \sum_{b \in V} \sum_{c \in V} Y^{1,*}_{a,\epsilon} Y^{2,*}_{i,\epsilon} Y^{3,*}_{b,\zeta} Y^{4,*}_{j,\zeta} {}^2D^{a,i,b,j} {}^2T_{c,k,a,i} V_{b,j,k,c} \quad (5864)$$

Factorized expression

$$\tau^0_{\gamma,\alpha,w} = \sum_{a \in V} {}^2D^3_{a,w} W^1_{a,\alpha} Y^{3,*}_{a,\gamma} \quad (3r_D r_T r_V N_v) \quad (5865)$$

$$\tau^1_{\gamma,\alpha,w} = \sum_{i \in O} {}^2D^4_{i,w} W^2_{i,\alpha} Y^{4,*}_{i,\gamma} \quad (3r_D r_T r_V N_o) \quad (5866)$$

$$\tau^2_{\gamma,\alpha} = \sum_{a \in V} W^4_{a,\alpha} Y^3_{a,\gamma} \quad (2r_T r_V N_v) \quad (5867)$$

$$\tau^3_{\gamma,\alpha} = \sum_{i \in O} W^3_{i,\alpha} Y^4_{i,\gamma} \quad (2r_T r_V N_o) \quad (5868)$$

$$\tau^4_{\gamma,\alpha} = \sum_{\beta \in B} X_{\alpha,\beta} \tau^2_{\gamma,\beta} \tau^3_{\gamma,\beta} \quad (3r_T r_V^2) \quad (5869)$$

$$\tau^5_{\gamma,\alpha} = \sum_{\delta \in A} Z_{\gamma,\delta} \tau^4_{\delta,\alpha} \quad (2r_T^2 r_V) \quad (5870)$$

$$\tau^6_{\gamma,\delta,w} = \sum_{\alpha \in B} \tau^5_{\gamma,\alpha} \tau^0_{\delta,\alpha,w} \tau^1_{\delta,\alpha,w} \quad (3r_D r_T^2 r_V) \quad (5871)$$

$$\tau^7_{\gamma,\delta,w} = \sum_{a \in V} {}^2D^1_{a,w} Y^1_{a,\gamma} Y^{1,*}_{a,\delta} \quad (3r_D r_T^2 N_v) \quad (5872)$$

$$\tau^8_{\gamma,\delta,w} = \sum_{i \in O} {}^2D^2_{i,w} Y^2_{i,\gamma} Y^{2,*}_{i,\delta} \quad (3r_D r_T^2 N_o) \quad (5873)$$

$${}^2R^z_{\epsilon,\gamma,\delta} \leftarrow \sum_{\epsilon \in A} \sum_{w \in D} \tau^6_{\epsilon,\delta,w} \tau^7_{\epsilon,\gamma,w} \tau^8_{\epsilon,\gamma,w} \quad (3r_D r_T^3) \quad (5874)$$

Raw expression

$${}^2R^z_{\epsilon,\zeta} \leftarrow \sum_{i \in O} \sum_{j \in O} \sum_{k \in O} \sum_{a \in V} \sum_{b \in V} \sum_{c \in V} Y^{1,*}_{a,\epsilon} Y^{2,*}_{i,\epsilon} Y^{3,*}_{b,\zeta} Y^{4,*}_{j,\zeta} {}^2D^{a,i,b,j} {}^2T_{c,k,b,j} V_{a,i,k,c} \quad (5875)$$

Factorized expression

$$\tau^0_{\gamma,\alpha,w} = \sum_{a \in V} {}^2D^3_{a,w} W^1_{a,\alpha} Y^{3,*}_{a,\gamma} \quad (3r_D r_T r_V N_v) \quad (5876)$$

$$\tau^1_{\gamma,\alpha,w} = \sum_{i \in O} {}^2D^4_{i,w} W^2_{i,\alpha} Y^{4,*}_{i,\gamma} \quad (3r_D r_T r_V N_o) \quad (5877)$$

$$\tau^2_{\gamma,\alpha} = \sum_{a \in V} W^4_{a,\alpha} Y^1_{a,\gamma} \quad (2r_T r_V N_v) \quad (5878)$$

$$\tau^3_{\gamma,\alpha} = \sum_{i \in O} W^3_{i,\alpha} Y^2_{i,\gamma} \quad (2r_T r_V N_o) \quad (5879)$$

$$\tau^4_{\gamma,\alpha} = \sum_{\beta \in B} X_{\alpha,\beta} \tau^2_{\gamma,\beta} \tau^3_{\gamma,\beta} \quad (3r_T r_V^2) \quad (5880)$$

$$\tau^5_{\gamma,\alpha} = \sum_{\delta \in A} Z_{\delta,\gamma} \tau^4_{\delta,\alpha} \quad (2r_T^2 r_V) \quad (5881)$$

$$\tau^6_{\gamma,\delta,w} = \sum_{\alpha \in B} \tau^5_{\gamma,\alpha} \tau^0_{\delta,\alpha,w} \tau^1_{\delta,\alpha,w} \quad (3r_D r_T^2 r_V) \quad (5882)$$

$$\tau^7_{\gamma,\delta,w} = \sum_{a \in V} {}^2D^1_{a,w} Y^3_{a,\gamma} Y^{1,*}_{a,\delta} \quad (3r_D r_T^2 N_v) \quad (5883)$$

$$\tau^8_{\gamma,\delta,w} = \sum_{i \in O} {}^2D^2_{i,w} Y^4_{i,\gamma} Y^{2,*}_{i,\delta} \quad (3r_D r_T^2 N_o) \quad (5884)$$

$${}^2R^z_{\gamma,\delta} \leftarrow \sum_{\epsilon \in A} \sum_{w \in D} \tau^6_{\epsilon,\delta,w} \tau^7_{\epsilon,\gamma,w} \tau^8_{\epsilon,\gamma,w} \quad (3r_D r_T^3) \quad (5885)$$

Raw expression

$${}^2R^z_{\epsilon,\zeta} \leftarrow - \sum_{i \in O} \sum_{j \in O} \sum_{k \in O} \sum_{a \in V} \sum_{b \in V} \sum_{c \in V} \frac{1}{2} Y^{1,*}_{a,\epsilon} Y^{2,*}_{i,\epsilon} Y^{3,*}_{b,\zeta} Y^{4,*}_{j,\zeta} {}^2D^{a,i,b,j} {}^2T_{a,i,c,k} V_{b,c,k,j} \quad (5886)$$

Factorized expression

$$\tau^0_{\alpha,i,j} = \sum_{\beta \in B} X_{\alpha,\beta} W^3_{i,\beta} W^4_{j,\beta} \quad (3r_V^2 N_o^2) \quad (5887)$$

$$\tau^1_{\gamma,\alpha,i} = \sum_{j \in O} Y^4_{j,\gamma} \tau^0_{\alpha,j,i} \quad (2r_T r_V N_o^2) \quad (5888)$$

$$\tau^2_{\gamma,\alpha} = \sum_{a \in V} W^2_{a,\alpha} Y^3_{a,\gamma} \quad (2r_T r_V N_v) \quad (5889)$$

$$\tau^3_{\gamma,i,a} = \sum_{\alpha \in B} W^1_{a,\alpha} \tau^2_{\gamma,\alpha} \tau^1_{\gamma,\alpha,i} \quad (3r_T r_V N_o N_v) \quad (5890)$$

$$\tau^4_{\gamma,\delta,w} = \sum_{i \in O} \sum_{a \in V} {}^2D^1_{a,w} {}^2D^2_{i,w} Y^{1,*}_{a,\delta} Y^{2,*}_{i,\delta} \tau^3_{\gamma,i,a} \quad (5r_D r_T^2 N_o N_v) \quad (5891)$$

$$\tau^5_{\gamma,\delta,w} = \sum_{a \in V} {}^2D^3_{a,w} Y^1_{a,\gamma} Y^{3,*}_{a,\delta} \quad (3r_D r_T^2 N_v) \quad (5892)$$

$$\tau^6_{\gamma,\delta,w} = \sum_{i \in O} {}^2D^4_{i,w} Y^2_{i,\gamma} Y^{4,*}_{i,\delta} \quad (3r_D r_T^2 N_o) \quad (5893)$$

$$\tau^7_{\gamma,\delta,w} = \sum_{\epsilon \in A} Z_{\epsilon,\gamma} \tau^5_{\epsilon,\delta,w} \tau^6_{\epsilon,\delta,w} \quad (3r_D r_T^3) \quad (5894)$$

$${}^2R^z_{\gamma,\delta} \leftarrow - \sum_{\epsilon \in A} \sum_{w \in D} \frac{1}{2} \tau^4_{\epsilon,\gamma,w} \tau^7_{\epsilon,\delta,w} \quad (2r_D r_T^3) \quad (5895)$$

Raw expression

$${}^2R^z_{\epsilon,\zeta} \leftarrow - \sum_{i \in O} \sum_{j \in O} \sum_{k \in O} \sum_{a \in V} \sum_{b \in V} \sum_{c \in V} \frac{1}{2} Y^{1,*}_{a,\epsilon} Y^{2,*}_{i,\epsilon} Y^{3,*}_{b,\zeta} Y^{4,*}_{j,\zeta} {}^2D^{a,i,b,j} {}^2T_{a,k,c,i} V_{b,j,k,c} \quad (5896)$$

Factorized expression

$$\tau^0_{\alpha,i,j} = \sum_{\beta \in B} X_{\alpha,\beta} W^3_{i,\beta} W^4_{j,\beta} \quad (3r_V^2 N_o^2) \quad (5897)$$

$$\tau^1_{\gamma,\alpha,i} = \sum_{j \in O} Y^2_{j,\gamma} \tau^0_{\alpha,j,i} \quad (2r_T r_V N_o^2) \quad (5898)$$

$$\tau^4_{\alpha,i,j} = \sum_{\beta \in B} X_{\alpha,\beta} W^3_{i,\beta} W^4_{j,\beta} \quad (3r_V^2 N_o^2) \quad (5911)$$

$$\tau^2_{\gamma,\alpha} = \sum_{a \in V} W^2_{a,\alpha} Y^1_{a,\gamma} \quad (2r_T r_V N_v) \quad (5899)$$

$$\tau^5_{\gamma,\alpha,i} = \sum_{j \in O} Y^2_{j,\gamma} \tau^4_{\alpha,j,i} \quad (2r_T r_V N_o^2) \quad (5912)$$

$$\tau^3_{\gamma,i,a} = \sum_{\alpha \in B} W^1_{a,\alpha} \tau^2_{\gamma,\alpha} \tau^1_{\gamma,\alpha,i} \quad (3r_T r_V N_o N_v) \quad (5900)$$

$$\tau^6_{\gamma,\delta,w,i} = \sum_{\alpha \in B} \tau^5_{\gamma,\alpha,i} \tau^3_{\gamma,\delta,\alpha,w} \quad (2r_D r_T^2 r_V N_o) \quad (5913)$$

$$\tau^4_{\gamma,\delta,w} = \sum_{i \in O} \sum_{a \in V} {}^2D^1_{a,w} {}^2D^2_{i,w} Y^{1,*}_{a,\delta} Y^{2,*}_{i,\delta} \tau^3_{\gamma,i,a} \quad (5r_D r_T^2 N_v N_o) \quad (5901)$$

$$\tau^7_{\gamma,\delta,w} = \sum_{i \in O} {}^2D^3_{a,w} Y^1_{a,\gamma} Y^{3,*}_{a,\delta} \quad (3r_D r_T^2 N_v) \quad (5914)$$

$$\tau^5_{\gamma,\delta,w} = \sum_{\epsilon \in A} Z_{\epsilon,\gamma} \tau^4_{\epsilon,\delta,w} \quad (2r_D r_T^3) \quad (5902)$$

$${}^2R^z_{\gamma,\delta} \leftarrow - \sum_{\epsilon \in A} \sum_{w \in D} \sum_{i \in O} \frac{1}{2} {}^2D^4_{i,w} Y^{4,*}_{i,\delta} \tau^7_{\epsilon,\delta,w} \tau^6_{\epsilon,\gamma,w,i} \quad (4r_D r_T^3 N_o) \quad (5915)$$

$$\tau^6_{\gamma,\delta,w} = \sum_{a \in V} {}^2D^3_{a,w} Y^3_{a,\gamma} Y^{3,*}_{a,\delta} \quad (3r_D r_T^2 N_v) \quad (5903)$$

Raw expression

$${}^2R^z_{\epsilon,\zeta} \leftarrow - \sum_{i \in O} \sum_{j \in O} \sum_{k \in O} \sum_{a \in V} \sum_{b \in V} \sum_{c \in V} \frac{1}{2} Y^{1,*}_{a,\epsilon} Y^{2,*}_{i,\epsilon} Y^{3,*}_{b,\zeta} Y^{4,*}_{j,\zeta} {}^2D^{a,i,b,j} {}^2T_{b,j,c,k} V_{a,c,k,i} \quad (5916)$$

$${}^2R^z_{\gamma,\delta} \leftarrow - \sum_{\epsilon \in A} \sum_{w \in D} \frac{1}{2} \tau^5_{\epsilon,\gamma,w} \tau^6_{\epsilon,\delta,w} \tau^7_{\epsilon,\delta,w} \quad (3r_D r_T^3) \quad (5905)$$

Factorized expression

$$\tau^0_{\gamma,\alpha,w} = \sum_{a \in V} {}^2D^1_{a,w} W^1_{a,\alpha} Y^{1,*}_{a,\gamma} \quad (3r_D r_T r_V N_v) \quad (5917)$$

Raw expression

$${}^2R^z_{\epsilon,\zeta} \leftarrow - \sum_{i \in O} \sum_{j \in O} \sum_{k \in O} \sum_{a \in V} \sum_{b \in V} \sum_{c \in V} \frac{1}{2} Y^{1,*}_{a,\epsilon} Y^{2,*}_{i,\epsilon} Y^{3,*}_{b,\zeta} Y^{4,*}_{j,\zeta} {}^2D^{a,i,b,j} {}^2T_{a,k,c,j} V_{b,c,k,i} \quad (5906)$$

Factorized expression

$$\tau^0_{\gamma,\alpha,w} = \sum_{a \in V} {}^2D^1_{a,w} W^1_{a,\alpha} Y^{1,*}_{a,\gamma} \quad (3r_D r_T r_V N_v) \quad (5907)$$

$$\tau^3_{\gamma,\delta,\alpha,w} = \sum_{i \in O} {}^2D^2_{i,w} Y^{2,*}_{i,\delta} \tau^0_{\delta,\alpha,w} \tau^2_{\gamma,\alpha,i} \quad (4r_D r_T^2 r_V N_o) \quad (5920)$$

$$\tau^1_{\gamma,\alpha} = \sum_{a \in V} W^2_{a,\alpha} Y^3_{a,\gamma} \quad (2r_T r_V N_v) \quad (5908)$$

$$\tau^4_{\alpha,i,j} = \sum_{\beta \in B} X_{\alpha,\beta} W^3_{i,\beta} W^4_{j,\beta} \quad (3r_V^2 N_o^2) \quad (5921)$$

$$\tau^2_{\gamma,\alpha,i} = \sum_{\delta \in A} Z_{\gamma,\delta} Y^4_{i,\delta} \tau^1_{\delta,\alpha} \quad (3r_T^2 r_V N_o) \quad (5909)$$

$$\tau^5_{\gamma,\alpha,i} = \sum_{j \in O} Y^4_{j,\gamma} \tau^4_{\alpha,j,i} \quad (2r_T r_V N_o^2) \quad (5922)$$

$$\tau^3_{\gamma,\delta,\alpha,w} = \sum_{i \in O} {}^2D^2_{i,w} Y^{2,*}_{i,\delta} \tau^0_{\delta,\alpha,w} \tau^2_{\gamma,\alpha,i} \quad (4r_D r_T^2 r_V N_o) \quad (5910)$$

$$\tau^6_{\gamma,\delta,w,i} = \sum_{\alpha \in B} \tau^5_{\gamma,\alpha,i} \tau^3_{\gamma,\delta,\alpha,w} \quad (2r_D r_T^2 r_V N_o) \quad (5923)$$



Raw expression

$$\tau_{\gamma,\delta,w}^7 = \sum_{a \in V} {}^2D_{a,w}^3 Y_{a,\gamma}^3 Y_{a,\delta}^{3,*} \quad (3r_D r_T^2 N_v) \quad (5924)$$

$${}^2R_{\gamma,\delta}^z \leftarrow - \sum_{\epsilon \in A} \sum_{w \in D} \sum_{i \in O} \frac{1}{2} {}^2D_{i,w}^4 Y_{i,\delta}^{4,*} \tau_{\epsilon,\delta,w}^7 \tau_{\epsilon,\gamma,w,i}^6 \quad (4r_D r_T^3 N_o) \quad (5925)$$

Raw expression

$${}^2R_{\epsilon,\zeta}^z \leftarrow - \sum_{i \in O} \sum_{j \in O} \sum_{k \in O} \sum_{a \in V} \sum_{b \in V} \sum_{c \in V} \frac{1}{2} Y_{a,\epsilon}^{1,*} Y_{i,\epsilon}^{2,*} Y_{b,\zeta}^{3,*} Y_{j,\zeta}^{4,*} {}^2D_{a,i,b,j} {}^2T_{b,k,c,i} V_{a,c,k,j} \quad (5926)$$

Factorized expression

$$\tau_{\gamma,\delta,w}^0 = \sum_{a \in V} {}^2D_{a,w}^3 Y_{a,\gamma}^1 Y_{a,\delta}^{3,*} \quad (3r_D r_T^2 N_v) \quad (5927)$$

$$\tau_{\gamma,\alpha}^1 = \sum_{i \in O} W_{i,\alpha}^3 Y_{i,\gamma}^2 \quad (2r_T r_V N_o) \quad (5928)$$

$$\tau_{\gamma,\alpha}^2 = \sum_{a \in V} W_{a,\alpha}^4 Y_{a,\gamma}^3 \quad (2r_T r_V N_v) \quad (5929)$$

$$\tau_{\gamma,\alpha,i}^3 = \sum_{\delta \in A} Z_{\gamma,\delta} Y_{i,\delta}^4 \tau_{\delta,\alpha}^2 \quad (3r_T^2 r_V N_o) \quad (5930)$$

$$\tau_{\gamma,\alpha,w}^4 = \sum_{\delta \in A} \sum_{i \in O} {}^2D_{i,w}^4 Y_{i,\gamma}^{4,*} \tau_{\delta,\alpha}^1 \tau_{\delta,\gamma,w}^0 \tau_{\delta,\alpha,i}^3 \quad (5r_D r_T^2 r_V N_o^6) \quad (5931)$$

$$\tau_{\gamma,\alpha,w}^5 = \sum_{\beta \in B} X_{\alpha,\beta} \tau_{\gamma,\beta,w}^4 \quad (2r_D r_T r_V^2) \quad (5932)$$

$$\tau_{\gamma,\alpha,w}^6 = \sum_{a \in V} {}^2D_{a,w}^1 W_{a,\alpha}^1 Y_{a,\gamma}^{1,*} \quad (3r_D r_T r_V N_v) \quad (5933)$$

$$\tau_{\gamma,\alpha,w}^7 = \sum_{i \in O} {}^2D_{i,w}^2 W_{i,\alpha}^2 Y_{i,\gamma}^{2,*} \quad (3r_D r_T r_V N_o) \quad (5934)$$

$${}^2R_{\gamma,\delta}^z \leftarrow - \sum_{\alpha \in B} \sum_{w \in D} \frac{1}{2} \tau_{\delta,\alpha,w}^5 \tau_{\gamma,\alpha,w}^6 \tau_{\gamma,\alpha,w}^7 \quad (3r_D r_T^2 r_V) \quad (5935)$$

$${}^2R_{\epsilon,\zeta}^z \leftarrow - \sum_{i \in O} \sum_{j \in O} \sum_{k \in O} \sum_{a \in V} \sum_{b \in V} \sum_{c \in V} \frac{1}{2} Y_{a,\epsilon}^{1,*} Y_{i,\epsilon}^{2,*} Y_{b,\zeta}^{3,*} Y_{j,\zeta}^{4,*} {}^2D_{a,i,b,j} {}^2T_{b,k,c,j} V_{a,i,k,c} \quad (5936)$$

Factorized expression

$$\tau_{\gamma,\delta,w}^0 = \sum_{a \in V} {}^2D_{a,w}^3 Y_{a,\gamma}^3 Y_{a,\delta}^{3,*} \quad (3r_D r_T^2 N_v) \quad (5937)$$

$$\tau_{\gamma,\alpha}^1 = \sum_{a \in V} W_{a,\alpha}^4 Y_{a,\gamma}^1 \quad (2r_T r_V N_v) \quad (5938)$$

$$\tau_{\gamma,\alpha,i}^2 = \sum_{\delta \in A} Y_{i,\delta}^2 Z_{\delta,\gamma} \tau_{\delta,\alpha}^1 \quad (3r_T^2 r_V N_o) \quad (5939)$$

$$\tau_{\gamma,\alpha}^3 = \sum_{i \in O} W_{i,\alpha}^3 Y_{i,\gamma}^4 \quad (2r_T r_V N_o) \quad (5940)$$

$$\tau_{\gamma,\alpha,w}^4 = \sum_{\delta \in A} \sum_{i \in O} {}^2D_{i,w}^4 Y_{i,\gamma}^{4,*} \tau_{\delta,\alpha}^3 \tau_{\delta,\gamma,w}^0 \tau_{\delta,\alpha,i}^2 \quad (5r_D r_T^2 r_V N_o) \quad (5941)$$

$$\tau_{\gamma,\alpha,w}^5 = \sum_{\beta \in B} X_{\alpha,\beta} \tau_{\gamma,\beta,w}^4 \quad (2r_D r_T r_V^2) \quad (5942)$$

$$\tau_{\gamma,\alpha,w}^7 = \sum_{i \in O} {}^2D_{i,w}^2 W_{i,\alpha}^2 Y_{i,\gamma}^{2,*} \quad (3r_D r_T r_V N_o) \quad (5944)$$

$${}^2R_{\gamma,\delta}^z \leftarrow - \sum_{\alpha \in B} \sum_{w \in D} \frac{1}{2} \tau_{\delta,\alpha,w}^5 \tau_{\gamma,\alpha,w}^6 \tau_{\gamma,\alpha,w}^7 \quad (3r_D r_T^2 r_V) \quad (5945)$$

Raw expression

$${}^2R_{\epsilon,\zeta}^z \leftarrow - \sum_{i \in O} \sum_{j \in O} \sum_{k \in O} \sum_{a \in V} \sum_{b \in V} \sum_{c \in V} \frac{1}{2} Y_{a,\epsilon}^{1,*} Y_{i,\epsilon}^{2,*} Y_{b,\zeta}^{3,*} Y_{j,\zeta}^{4,*} {}^2D_{a,i,b,j} {}^2T_{c,i,a,k} V_{b,j,k,c} \quad (5946)$$

Factorized expression

$$\tau_{\gamma,\delta,w}^0 = \sum_{a \in V} {}^2D^1_{a,w} Y^1_{a,\gamma} Y^{1,*}_{a,\delta} \quad (3r_D r_T^2 N_v) \quad (5947)$$

$$\tau_{\gamma,\alpha}^2 = \sum_{a \in V} W^2_{a,\alpha} Y^1_{a,\gamma} \quad (2r_T r_V N_v) \quad (5959)$$

$$\tau_{\gamma,\alpha,w}^1 = \sum_{a \in V} {}^2D^3_{a,w} W^1_{a,\alpha} Y^{3,*}_{a,\gamma} \quad (3r_D r_T r_V N_v) \quad (5948)$$

$$\tau_{\gamma,\alpha,i}^3 = \sum_{\delta \in A} Y^2_{i,\delta} Z_{\delta,\gamma} \tau_{\delta,\alpha}^2 \quad (3r_T^2 r_V N_o) \quad (5960)$$

$$\tau_{\gamma,\alpha}^2 = \sum_{a \in V} W^2_{a,\alpha} Y^3_{a,\gamma} \quad (2r_T r_V N_v) \quad (5949)$$

$$\tau_{\gamma,\delta,\alpha,w}^4 = \sum_{i \in O} {}^2D^4_{i,w} Y^{4,*}_{i,\delta} \tau_{\delta,\alpha,w}^1 \tau_{\gamma,\alpha,i}^3 \quad (4r_D r_T^2 r_V N_o) \quad (5961)$$

$$\tau_{\gamma,\alpha,i}^3 = \sum_{\delta \in A} Z_{\gamma,\delta} Y^4_{i,\delta} \tau_{\delta,\alpha}^2 \quad (3r_T^2 r_V N_o) \quad (5950)$$

$$\tau_{\alpha,i,j}^5 = \sum_{\beta \in B} X_{\alpha,\beta} W^3_{i,\beta} W^4_{j,\beta} \quad (3r_V^2 N_o^2) \quad (5962)$$

$$\tau_{\gamma,\delta,\alpha,w}^4 = \sum_{i \in O} {}^2D^4_{i,w} Y^{4,*}_{i,\delta} \tau_{\delta,\alpha,w}^1 \tau_{\gamma,\alpha,i}^3 \quad (4r_D r_T^2 r_V N_o) \quad (5951)$$

$$\tau_{\gamma,\alpha,i}^6 = \sum_{j \in O} Y^4_{j,\gamma} \tau_{\alpha,j,i}^5 \quad (2r_T r_V N_o^2) \quad (5963)$$

$$\tau_{\alpha,i,j}^5 = \sum_{\beta \in B} X_{\alpha,\beta} W^3_{i,\beta} W^4_{j,\beta} \quad (3r_V^2 N_o^2) \quad (5952)$$

$$\tau_{\gamma,\delta,w,i}^7 = \sum_{\alpha \in B} \tau_{\gamma,\alpha,i}^6 \tau_{\gamma,\delta,\alpha,w}^4 \quad (2r_D r_T^2 r_V N_o) \quad (5964)$$

$$\tau_{\gamma,\alpha,i}^6 = \sum_{j \in O} Y^2_{j,\gamma} \tau_{\alpha,j,i}^5 \quad (2r_T r_V N_o^2) \quad (5953)$$

$${}^2R^z_{\gamma,\delta} \leftarrow - \sum_{\epsilon \in A} \sum_{w \in D} \sum_{i \in O} \frac{1}{2} {}^2D^2_{i,w} Y^{2,*}_{i,\gamma} \tau_{\epsilon,\gamma,w}^0 \tau_{\epsilon,\delta,w,i}^7 \quad (4r_D r_T^3 N_o) \quad (5965)$$

Raw expression

$$\tau_{\gamma,\delta,w,i}^7 = \sum_{\alpha \in B} \tau_{\gamma,\alpha,i}^6 \tau_{\gamma,\delta,\alpha,w}^4 \quad (2r_D r_T^2 r_V N_o) \quad (5954)$$

$${}^2R^z_{\epsilon,\zeta} \leftarrow - \sum_{i \in O} \sum_{j \in O} \sum_{k \in O} \sum_{a \in V} \sum_{b \in V} \sum_{c \in V} \frac{1}{2} Y^{1,*}_{a,\epsilon} Y^{2,*}_{i,\epsilon} Y^{3,*}_{b,\zeta} Y^{4,*}_{j,\zeta} {}^2D^{a,i,b,j} T_{c,j,a,k} V_{b,c,k,i} \quad (5966)$$

$${}^2R^z_{\gamma,\delta} \leftarrow - \sum_{\epsilon \in A} \sum_{w \in D} \sum_{i \in O} \frac{1}{2} {}^2D^2_{i,w} Y^{2,*}_{i,\gamma} \tau_{\epsilon,\gamma,w}^0 \tau_{\epsilon,\delta,w,i}^7 \quad (4r_D r_T^3 N_o) \quad (5955)$$

Factorized expression

Raw expression

$${}^2R^z_{\epsilon,\zeta} \leftarrow - \sum_{i \in O} \sum_{j \in O} \sum_{k \in O} \sum_{a \in V} \sum_{b \in V} \sum_{c \in V} \frac{1}{2} Y^{1,*}_{a,\epsilon} Y^{2,*}_{i,\epsilon} Y^{3,*}_{b,\zeta} Y^{4,*}_{j,\zeta} {}^2D^{a,i,b,j} T_{c,i,b,k} V_{a,c,k,j} \quad (5956)$$

Factorized expression

$$\tau_{\gamma,\delta,w}^0 = \sum_{a \in V} {}^2D^1_{a,w} Y^3_{a,\gamma} Y^{1,*}_{a,\delta} \quad (3r_D r_T^2 N_v) \quad (5957)$$

$$\tau_{\gamma,\delta,w}^0 = \sum_{a \in V} {}^2D^1_{a,w} Y^1_{a,\gamma} Y^{1,*}_{a,\delta} \quad (3r_D r_T^2 N_v) \quad (5967)$$

$$\tau_{\gamma,\delta,w}^1 = \sum_{i \in O} {}^2D^2_{i,w} Y^2_{i,\gamma} Y^{2,*}_{i,\delta} \quad (3r_D r_T^2 N_o) \quad (5968)$$

$$\tau_{\gamma,\delta,w}^2 = \sum_{\epsilon \in A} Z_{\epsilon,\gamma} \tau_{\epsilon,\delta,w}^0 \tau_{\epsilon,\delta,w}^1 \quad (3r_D r_T^3) \quad (5969)$$

$$\tau_{\alpha,i,j}^3 = \sum_{\beta \in B} X_{\alpha,\beta} W^3_{i,\beta} W^4_{j,\beta} \quad (3r_V^2 N_o^2) \quad (5970)$$

$$\tau_{\gamma,\alpha,w}^1 = \sum_{a \in V} {}^2D^3_{a,w} W^1_{a,\alpha} Y^{3,*}_{a,\gamma} \quad (3r_D r_T r_V N_v) \quad (5958)$$

$$\tau_{\gamma,\alpha,i}^4 = \sum_{j \in O} Y^4_{j,\gamma} \tau_{\alpha,j,i}^3 \quad (2r_T r_V N_o^2) \quad (5971)$$

$$\tau^5_{\gamma,\alpha} = \sum_{a \in V} W^2_{a,\alpha} Y^3_{a,\gamma} \quad (2r_T r_V N_v) \quad (5972)$$

$${}^2R^z_{\gamma,\delta} \leftarrow - \sum_{\epsilon \in A} \sum_{w \in D} \frac{1}{2} \tau^0_{\epsilon,\gamma,w} \tau^1_{\epsilon,\gamma,w} \tau^7_{\epsilon,\delta,w} \quad (3r_D r_T^3) \quad (5985)$$

$$\tau^6_{\gamma,i,a} = \sum_{\alpha \in B} W^1_{a,\alpha} \tau^5_{\gamma,\alpha} \tau^4_{\gamma,\alpha,i} \quad (3r_T r_V N_o N_v) \quad (5973)$$

Raw expression

$$\tau^7_{\gamma,\delta,w} = \sum_{i \in O} \sum_{a \in V} {}^2D^3_{a,w} {}^2D^4_{i,w} Y^{3,*}_{a,\delta} Y^{4,*}_{i,\delta} \tau^6_{\gamma,i,a} \quad (5r_D r_T^2 N_o N_v) \quad (5974)$$

$${}^2R^z_{\epsilon,\zeta} \leftarrow - \sum_{i \in O} \sum_{j \in O} \sum_{k \in O} \sum_{a \in V} \sum_{b \in V} \sum_{c \in V} \frac{1}{2} Y^{1,*}_{a,\epsilon} Y^{2,*}_{i,\epsilon} Y^{3,*}_{b,\zeta} Y^{4,*}_{j,\zeta} {}^2D^{a,i,b,j} {}^2T_{c,k,a,i} V_{b,c,k,j} \quad (5986)$$

$${}^2R^z_{\gamma,\delta} \leftarrow - \sum_{\epsilon \in A} \sum_{w \in D} \frac{1}{2} \tau^2_{\epsilon,\gamma,w} \tau^7_{\epsilon,\delta,w} \quad (2r_D r_T^3) \quad (5975)$$

Factorized expression

Raw expression

$${}^2R^z_{\epsilon,\zeta} \leftarrow - \sum_{i \in O} \sum_{j \in O} \sum_{k \in O} \sum_{a \in V} \sum_{b \in V} \sum_{c \in V} \frac{1}{2} Y^{1,*}_{a,\epsilon} Y^{2,*}_{i,\epsilon} Y^{3,*}_{b,\zeta} Y^{4,*}_{j,\zeta} {}^2D^{a,i,b,j} {}^2T_{c,j,b,k} V_{a,i,k,c} \quad (5976)$$

$$\tau^0_{\gamma,\alpha,w} = \sum_{a \in V} {}^2D^3_{a,w} W^1_{a,\alpha} Y^{3,*}_{a,\gamma} \quad (3r_D r_T r_V N_v) \quad (5987)$$

$$\tau^1_{\gamma,\alpha,w} = \sum_{i \in O} {}^2D^4_{i,w} W^2_{i,\alpha} Y^{4,*}_{i,\gamma} \quad (3r_D r_T r_V N_o) \quad (5988)$$

Factorized expression

$$\tau^0_{\gamma,\delta,w} = \sum_{a \in V} {}^2D^1_{a,w} Y^3_{a,\gamma} Y^{1,*}_{a,\delta} \quad (3r_D r_T^2 N_v) \quad (5977)$$

$$\tau^2_{\gamma,\delta,w} = \sum_{a \in V} {}^2D^1_{a,w} Y^1_{a,\gamma} Y^{1,*}_{a,\delta} \quad (3r_D r_T^2 N_v) \quad (5989)$$

$$\tau^1_{\gamma,\delta,w} = \sum_{i \in O} {}^2D^2_{i,w} Y^4_{i,\gamma} Y^{2,*}_{i,\delta} \quad (3r_D r_T^2 N_o) \quad (5978)$$

$$\tau^3_{\gamma,\alpha} = \sum_{i \in O} W^3_{i,\alpha} Y^2_{i,\gamma} \quad (2r_T r_V N_o) \quad (5990)$$

$$\tau^2_{\alpha,i,j} = \sum_{\beta \in B} X_{\alpha,\beta} W^3_{i,\beta} W^4_{j,\beta} \quad (3r_V^2 N_o^2) \quad (5979)$$

$$\tau^4_{\gamma,\alpha} = \sum_{a \in V} W^4_{a,\alpha} Y^3_{a,\gamma} \quad (2r_T r_V N_v) \quad (5991)$$

$$\tau^3_{\gamma,\alpha,i} = \sum_{j \in O} Y^2_{j,\gamma} \tau^2_{\alpha,j,i} \quad (2r_T r_V N_o^2) \quad (5980)$$

$$\tau^5_{\gamma,\alpha,i} = \sum_{\delta \in A} Z_{\gamma,\delta} Y^4_{i,\delta} \tau^4_{\delta,\alpha} \quad (3r_T^2 r_V N_o) \quad (5992)$$

$$\tau^4_{\gamma,\alpha} = \sum_{a \in V} W^2_{a,\alpha} Y^1_{a,\gamma} \quad (2r_T r_V N_v) \quad (5981)$$

$$\tau^6_{\gamma,\alpha,w} = \sum_{\delta \in A} \sum_{i \in O} {}^2D^2_{i,w} Y^{2,*}_{i,\gamma} \tau^3_{\delta,\alpha} \tau^2_{\delta,\gamma,w} \tau^5_{\delta,\alpha,i} \quad (5r_D r_T^2 r_V N_o) \quad (5993)$$

$$\tau^5_{\gamma,i,a} = \sum_{\alpha \in B} W^1_{a,\alpha} \tau^4_{\gamma,\alpha} \tau^3_{\gamma,\alpha,i} \quad (3r_T r_V N_o N_v) \quad (5982)$$

$$\tau^7_{\gamma,\alpha,w} = \sum_{\beta \in B} X_{\alpha,\beta} \tau^6_{\gamma,\beta,w} \quad (2r_D r_T r_V^2) \quad (5994)$$

$$\tau^6_{\gamma,\delta,w} = \sum_{i \in O} \sum_{a \in V} {}^2D^3_{a,w} {}^2D^4_{i,w} Y^{3,*}_{a,\delta} Y^{4,*}_{i,\delta} \tau^5_{\gamma,i,a} \quad (5r_D r_T^2 N_o N_v) \quad (5983)$$

$${}^2R^z_{\gamma,\delta} \leftarrow - \sum_{\alpha \in B} \sum_{w \in D} \frac{1}{2} \tau^0_{\delta,\alpha,w} \tau^1_{\delta,\alpha,w} \tau^7_{\gamma,\alpha,w} \quad (3r_D r_T^2 r_V) \quad (5995)$$

$$\tau^7_{\gamma,\delta,w} = \sum_{\epsilon \in A} Z_{\epsilon,\gamma} \tau^6_{\epsilon,\delta,w} \quad (2r_D r_T^3) \quad (5984)$$

Raw expression

$${}^2R^z_{\epsilon,\zeta} \leftarrow - \sum_{i \in O} \sum_{j \in O} \sum_{k \in O} \sum_{a \in V} \sum_{b \in V} \sum_{c \in V} \frac{1}{2} Y^{1,*}_{a,\epsilon} Y^{2,*}_{i,\epsilon} Y^{3,*}_{b,\zeta} Y^{4,*}_{j,\zeta} {}^2D^{a,i,b,j} {}^2T_{c,k,b,j} V_{a,c,k,i} \quad (5996)$$

Factorized expression

$$\tau^0_{\gamma,\alpha,w} = \sum_{a \in V} {}^2D^3_{a,w} W^1_{a,\alpha} Y^{3,*}_{a,\gamma} \quad (3r_D r_T r_V N_v) \quad (5997)$$

$$\tau^1_{\gamma,\alpha,w} = \sum_{i \in O} {}^2D^4_{i,w} W^2_{i,\alpha} Y^{4,*}_{i,\gamma} \quad (3r_D r_T r_V N_o) \quad (5998)$$

$$\tau^2_{\gamma,\delta,w} = \sum_{a \in V} {}^2D^1_{a,w} Y^3_{a,\gamma} Y^{1,*}_{a,\delta} \quad (3r_D r_T^2 N_v) \quad (5999)$$

$$\tau^3_{\gamma,\alpha} = \sum_{a \in V} W^4_{a,\alpha} Y^1_{a,\gamma} \quad (2r_T r_V N_v) \quad (6000)$$

$$\tau^4_{\gamma,\alpha,i} = \sum_{\delta \in A} Y^2_{i,\delta} Z_{\delta,\gamma} \tau^3_{\delta,\alpha} \quad (3r_T^2 r_V N_o) \quad (6001)$$

$$\tau^5_{\gamma,\alpha} = \sum_{i \in O} W^3_{i,\alpha} Y^4_{i,\gamma} \quad (2r_T r_V N_o) \quad (6002)$$

$$\tau^6_{\gamma,\alpha,w} = \sum_{\delta \in A} \sum_{i \in O} {}^2D^2_{i,w} Y^{2,*}_{i,\gamma} \tau^5_{\delta,\alpha} \tau^2_{\delta,\gamma,w} \tau^4_{\delta,\alpha,i} \quad (5r_D r_T^2 r_V N_o) \quad (6003)$$

$$\tau^7_{\gamma,\alpha,w} = \sum_{\beta \in B} X_{\alpha,\beta} \tau^6_{\gamma,\beta,w} \quad (2r_D r_T r_V^2) \quad (6004)$$

$${}^2R^z_{\gamma,\delta} \leftarrow - \sum_{\alpha \in B} \sum_{w \in D} \frac{1}{2} \tau^0_{\delta,\alpha,w} \tau^1_{\delta,\alpha,w} \tau^7_{\gamma,\alpha,w} \quad (3r_D r_T^2 r_V) \quad (6005)$$

Raw expression

$${}^2R^z_{\epsilon,\zeta} \leftarrow \sum_{i \in O} \sum_{j \in O} \sum_{k \in O} \sum_{l \in O} \sum_{a \in V} \sum_{b \in V} \frac{1}{2} Y^{1,*}_{a,\epsilon} Y^{2,*}_{i,\epsilon} Y^{3,*}_{b,\zeta} Y^{4,*}_{j,\zeta} {}^2D^{a,i,b,j} {}^2T_{a,k,b,l} V_{k,i,l,j} \quad (6006)$$

Factorized expression

$$\tau^0_{\gamma,\alpha,w} = \sum_{a \in V} {}^2D^1_{a,w} W^1_{a,\alpha} Y^{1,*}_{a,\gamma} \quad (3r_D r_T r_V N_v) \quad (6007)$$

$$\tau^1_{\gamma,\alpha} = \sum_{a \in V} W^2_{a,\alpha} Y^1_{a,\gamma} \quad (2r_T r_V N_v) \quad (6008)$$

$$\tau^2_{\gamma,\alpha,i} = \sum_{\delta \in A} Y^2_{i,\delta} Z_{\delta,\gamma} \tau^1_{\delta,\alpha} \quad (3r_T^2 r_V N_o) \quad (6009)$$

$$\tau^3_{\gamma,\delta,\alpha,w} = \sum_{i \in O} {}^2D^2_{i,w} Y^{2,*}_{i,\delta} \tau^0_{\delta,\alpha,w} \tau^2_{\gamma,\alpha,i} \quad (4r_D r_T^2 r_V N_o) \quad (6010)$$

$$\tau^4_{\gamma,\alpha} = \sum_{a \in V} W^4_{a,\alpha} Y^3_{a,\gamma} \quad (2r_T r_V N_v) \quad (6011)$$

$$\tau^5_{\gamma,\alpha,a} = \sum_{\beta \in B} X_{\alpha,\beta} W^3_{a,\beta} \tau^4_{\gamma,\beta} \quad (3r_T r_V^2 N_v) \quad (6012)$$

$$\tau^6_{\gamma,\delta,w,a} = \sum_{\alpha \in B} \tau^5_{\gamma,\alpha,a} \tau^3_{\gamma,\delta,\alpha,w} \quad (2r_D r_T^2 r_V N_v) \quad (6013)$$

$$\tau^7_{\gamma,i,a} = \sum_{\delta \in A} \sum_{w \in D} {}^2D^3_{a,w} {}^2D^4_{i,w} Y^4_{i,\delta} \tau^6_{\delta,\gamma,w,a} \quad (4r_D r_T^2 N_o N_v) \quad (6014)$$

$$\tau^7_{\gamma,\alpha,w} \leftarrow \sum_{i \in O} \sum_{a \in V} \frac{1}{2} Y^{3,*}_{a,\delta} Y^{4,*}_{i,\delta} \tau^7_{\gamma,i,a} \quad (3r_T^2 N_o N_v) \quad (6015)$$

Raw expression

$${}^2R^z_{\epsilon,\zeta} \leftarrow \sum_{i \in O} \sum_{j \in O} \sum_{k \in O} \sum_{l \in O} \sum_{a \in V} \sum_{b \in V} \frac{1}{2} Y^{1,*}_{a,\epsilon} Y^{2,*}_{i,\epsilon} Y^{3,*}_{b,\zeta} Y^{4,*}_{j,\zeta} {}^2D^{a,i,b,j} {}^2T_{b,k,a,l} V_{l,i,k,j} \quad (6016)$$

Factorized expression

$$\tau^0_{\gamma,\alpha,w} = \sum_{a \in V} {}^2D^1_{a,w} W^1_{a,\alpha} Y^{1,*}_{a,\gamma} \quad (3r_D r_T r_V N_v) \quad (6017)$$

$$\tau^1_{\gamma,\alpha} = \sum_{a \in V} W^2_{a,\alpha} Y^3_{a,\gamma} \quad (2r_T r_V N_v) \quad (6018)$$

$$\tau^2_{\gamma,\alpha,i} = \sum_{\delta \in A} Z_{\gamma,\delta} Y^4_{i,\delta} \tau^1_{\delta,\alpha} \quad (3r_T^2 r_V N_o) \quad (6019)$$

$$\tau^3_{\gamma,\delta,\alpha,w} = \sum_{i \in O} {}^2D^2_{i,w} Y^{2,*}_{i,\delta} \tau^0_{\delta,\alpha,w} \tau^2_{\gamma,\alpha,i} \quad (4r_D r_T^2 r_V N_o) \quad (6020)$$

$$\tau^4_{\gamma,\alpha} = \sum_{a \in V} W^4_{a,\alpha} Y^1_{a,\gamma} \quad (2r_T r_V N_v) \quad (6021)$$

$$\tau^5_{\gamma,\alpha,a} = \sum_{\beta \in B} X_{\alpha,\beta} W^3_{a,\beta} \tau^4_{\gamma,\beta} \quad (3r_T r_V^2 N_v) \quad (6022)$$

$$\tau^6_{\gamma,\delta,w,a} = \sum_{\alpha \in B} \tau^5_{\gamma,\alpha,a} \tau^3_{\gamma,\delta,\alpha,w} \quad (2r_D r_T^2 r_V N_v) \quad (6023)$$

$$\tau^7_{\gamma,i,a} = \sum_{\delta \in A} \sum_{w \in D} {}^2D^3_{a,w} {}^2D^4_{i,w} Y^2_{i,\delta} \tau^6_{\delta,\gamma,w,a} \quad (4r_D r_T^2 N_o N_v) \quad (6024)$$

$${}^2R^z_{\gamma,\delta} \leftarrow \sum_{i \in O} \sum_{a \in V} \frac{1}{2} Y^{3,*}_{a,\delta} Y^{4,*}_{i,\delta} \tau^7_{\gamma,i,a} \quad (3r_T^2 N_o N_v) \quad (6025)$$

Raw expression

$${}^2R^z_{\epsilon,\zeta} \leftarrow \sum_{i \in O} \sum_{j \in O} \sum_{a \in V} \sum_{b \in V} \sum_{c \in V} \sum_{d \in V} \frac{1}{2} Y^{1,*}_{a,\epsilon} Y^{2,*}_{i,\epsilon} Y^{3,*}_{b,\zeta} Y^{4,*}_{j,\zeta} {}^2D^{a,i,b,j} {}^2T_{c,i,d,j} V_{a,c,b,d} \quad (6026)$$

Factorized expression

$$\tau^0_{\gamma,\delta,w} = \sum_{a \in V} {}^2D^3_{a,w} Y^3_{a,\gamma} Y^{3,*}_{a,\delta} \quad (3r_D r_T^2 N_v) \quad (6027)$$

$$\tau^1_{\gamma,i} = \sum_{j \in O} Y^4_{j,\gamma} f_{j,i} \quad (2r_T N_o^2) \quad (6028)$$

$$\tau^2_{\gamma,\delta,w} = \sum_{i \in O} {}^2D^4_{i,w} Y^{4,*}_{i,\delta} \tau^1_{\gamma,i} \quad (3r_D r_T^2 N_o) \quad (6029)$$

$$\tau^3_{\gamma,\delta,w} = \sum_{a \in V} {}^2D^1_{a,w} Y^1_{a,\gamma} Y^{1,*}_{a,\delta} \quad (3r_D r_T^2 N_v) \quad (6030)$$

$$\tau^4_{\gamma,\delta,w} = \sum_{i \in O} {}^2D^2_{i,w} Y^2_{i,\gamma} Y^{2,*}_{i,\delta} \quad (3r_D r_T^2 N_o) \quad (6031)$$

$$\tau^5_{\gamma,\delta,w} = \sum_{\epsilon \in A} Z_{\epsilon,\gamma} \tau^3_{\epsilon,\delta,w} \tau^4_{\epsilon,\delta,w} \quad (3r_D r_T^3) \quad (6032)$$

$${}^2R^z_{\gamma,\delta} \leftarrow - \sum_{\epsilon \in A} \sum_{w \in D} \frac{1}{2} \tau^0_{\epsilon,\delta,w} \tau^2_{\epsilon,\delta,w} \tau^5_{\epsilon,\gamma,w} \quad (3r_D r_T^3) \quad (6033)$$

Raw expression

$${}^2R^z_{\epsilon,\zeta} \leftarrow \sum_{i \in O} \sum_{j \in O} \sum_{a \in V} \sum_{b \in V} \sum_{c \in V} \sum_{d \in V} \frac{1}{2} Y^{1,*}_{a,\epsilon} Y^{2,*}_{i,\epsilon} Y^{3,*}_{b,\zeta} Y^{4,*}_{j,\zeta} {}^2D^{a,i,b,j} {}^2T_{c,j,d,i} V_{a,d,b,c} \quad (6034)$$

Factorized expression

$$\tau^0_{\gamma,\delta,w} = \sum_{a \in V} {}^2D^3_{a,w} Y^3_{a,\gamma} Y^{3,*}_{a,\delta} \quad (3r_D r_T^2 N_v) \quad (6035)$$

$$\tau^1_{\gamma,\delta,w} = \sum_{i \in O} {}^2D^4_{i,w} Y^4_{i,\gamma} Y^{4,*}_{i,\delta} \quad (3r_D r_T^2 N_o) \quad (6036)$$

$$\tau^2_{\gamma,\delta,w} = \sum_{a \in V} {}^2D^1_{a,w} Y^1_{a,\gamma} Y^{1,*}_{a,\delta} \quad (3r_D r_T^2 N_v) \quad (6037)$$

$$\tau^3_{\gamma,i} = \sum_{j \in O} Y^2_{j,\gamma} f_{j,i} \quad (2r_T N_o^2) \quad (6038)$$

$$\tau^4_{\gamma,\delta,w} = \sum_{i \in O} {}^2D^2_{i,w} Y^{2,*}_{i,\delta} \tau^3_{\gamma,i} \quad (3r_D r_T^2 N_o) \quad (6039)$$

$$\tau^5_{\gamma,\delta,w} = \sum_{\epsilon \in A} Z_{\epsilon,\gamma} \tau^2_{\epsilon,\delta,w} \tau^4_{\epsilon,\delta,w} \quad (3r_D r_T^3) \quad (6040)$$

$${}^2R^z_{\gamma,\delta} \leftarrow - \sum_{\epsilon \in A} \sum_{w \in D} \frac{1}{2} \tau^0_{\epsilon,\delta,w} \tau^1_{\epsilon,\delta,w} \tau^5_{\epsilon,\gamma,w} \quad (3r_D r_T^3) \quad (6041)$$

Raw expression

$${}^2R^z_{\epsilon,\zeta} \leftarrow \sum_{i \in O} \sum_{j \in O} \sum_{a \in V} \sum_{b \in V} \sum_{c \in V} \frac{1}{2} Y^{1,*}_{a,\epsilon} Y^{2,*}_{i,\epsilon} Y^{3,*}_{b,\zeta} Y^{4,*}_{j,\zeta} f_{a,c} {}^2D^{a,i,b,j} {}^2T_{b,j,c,i} \quad (6042)$$

Factorized expression

$$\tau^0_{\gamma,\delta,w} = \sum_{a \in V} {}^2D^3_{a,w} Y^1_{a,\gamma} Y^{3,*}_{a,\delta} \quad (3r_D r_T^2 N_v) \quad (6043)$$

$$\tau^1_{\gamma,\delta,w} = \sum_{i \in O} {}^2D^4_{i,w} Y^2_{i,\gamma} Y^{4,*}_{i,\delta} \quad (3r_D r_T^2 N_o) \quad (6044)$$

$$\tau^2_{\gamma,\delta,w} = \sum_{\epsilon \in A} Z_{\epsilon,\gamma} \tau^0_{\epsilon,\delta,w} \tau^1_{\epsilon,\delta,w} \quad (3r_D r_T^3) \quad (6045)$$

$$\tau^3_{\gamma,\delta,w} = \sum_{a \in V} {}^2D^1_{a,w} Y^3_{a,\gamma} Y^{1,*}_{a,\delta} \quad (3r_D r_T^2 N_v) \quad (6046)$$

$$\tau^4_{\gamma,i} = \sum_{j \in O} Y^4_{j,\gamma} f_{j,i} \quad (2r_T N_o^2) \quad (6047)$$

$$\tau^5_{\gamma,\delta,w} = \sum_{i \in O} {}^2D^2_{i,w} Y^{2,*}_{i,\delta} \tau^4_{\gamma,i} \quad (3r_D r_T^2 N_o) \quad (6048)$$

$${}^2R^z_{\gamma,\delta} \leftarrow - \sum_{\epsilon \in A} \sum_{w \in D} \frac{1}{2} \tau^2_{\epsilon,\delta,w} \tau^3_{\epsilon,\gamma,w} \tau^5_{\epsilon,\gamma,w} \quad (3r_D r_T^3) \quad (6049)$$

Raw expression

$${}^2R^z_{\epsilon,\zeta} \leftarrow \sum_{i \in O} \sum_{j \in O} \sum_{a \in V} \sum_{b \in V} \sum_{c \in V} \frac{1}{2} Y^{1,*}_{a,\epsilon} Y^{2,*}_{i,\epsilon} Y^{3,*}_{b,\zeta} Y^{4,*}_{j,\zeta} f_{a,c} {}^2D^{a,i,b,j} {}^2T_{c,i,b,j} \quad (6050)$$

Factorized expression

$$\tau^0_{\gamma,\delta,w} = \sum_{a \in V} {}^2D^3_{a,w} Y^1_{a,\gamma} Y^{3,*}_{a,\delta} \quad (3r_D r_T^2 N_v) \quad (6051)$$

$$\tau^1_{\gamma,i} = \sum_{j \in O} Y^2_{j,\gamma} f_{j,i} \quad (2r_T N_o^2) \quad (6052)$$

$$\tau^2_{\gamma,\delta,w} = \sum_{i \in O} {}^2D^4_{i,w} Y^{4,*}_{i,\delta} \tau^1_{\gamma,i} \quad (3r_D r_T^2 N_o) \quad (6053)$$

$$\tau^3_{\gamma,\delta,w} = \sum_{\epsilon \in A} Z_{\epsilon,\gamma} \tau^0_{\epsilon,\delta,w} \tau^2_{\epsilon,\delta,w} \quad (3r_D r_T^3) \quad (6054)$$

$$\tau^4_{\gamma,\delta,w} = \sum_{a \in V} {}^2D^1_{a,w} Y^3_{a,\gamma} Y^{1,*}_{a,\delta} \quad (3r_D r_T^2 N_v) \quad (6055)$$

$$\tau^5_{\gamma,\delta,w} = \sum_{i \in O} {}^2D^2_{i,w} Y^4_{i,\gamma} Y^{2,*}_{i,\delta} \quad (3r_D r_T^2 N_o) \quad (6056)$$

$${}^2R^z_{\gamma,\delta} \leftarrow - \sum_{\epsilon \in A} \sum_{w \in D} \frac{1}{2} \tau^3_{\epsilon,\delta,w} \tau^4_{\epsilon,\gamma,w} \tau^5_{\epsilon,\gamma,w} \quad (3r_D r_T^3) \quad (6057)$$

Raw expression

$${}^2R^z_{\epsilon,\zeta} \leftarrow \sum_{i \in O} \sum_{j \in O} \sum_{a \in V} \sum_{b \in V} \sum_{c \in V} \frac{1}{2} Y^{1,*}_{a,\epsilon} Y^{2,*}_{i,\epsilon} Y^{3,*}_{b,\zeta} Y^{4,*}_{j,\zeta} f_{b,c} {}^2D^{a,i,b,j} {}^2T_{a,i,c,j} \quad (6058)$$

Factorized expression

$$\tau^0_{\gamma,\alpha,w} = \sum_{i \in O} {}^2D^4_{i,w} W^4_{i,\alpha} Y^{4,*}_{i,\gamma} \quad (3r_D r_T r_V N_o) \quad (6059)$$

$$\tau^1_{\gamma,\delta,w} = \sum_{a \in V} {}^2D^3_{a,w} Y^3_{a,\gamma} Y^{3,*}_{a,\delta} \quad (3r_D r_T^2 N_v) \quad (6060)$$

$$\tau^2_{\gamma,\delta,w,i} = \sum_{\epsilon \in A} Z_{\gamma,\epsilon} Y^4_{i,\epsilon} \tau^1_{\epsilon,\delta,w} \quad (3r_D r_T^3 N_o) \quad (6061)$$

$$\tau^3_{\gamma,\delta,\alpha,w} = \sum_{i \in O} W^3_{i,\alpha} \tau^0_{\delta,\alpha,w} \tau^2_{\gamma,\delta,w,i} \quad (3r_D r_T^2 r_V N_o) \quad (6062)$$

$$\tau^4_{\alpha,i,j} = \sum_{\beta \in B} W^1_{i,\beta} W^2_{j,\beta} X_{\beta,\alpha} \quad (3r_V^2 N_o^2) \quad (6063)$$

$$\tau^5_{\gamma,\alpha,i} = \sum_{j \in O} Y^2_{j,\gamma} \tau^4_{\alpha,j,i} \quad (2r_T r_V N_o^2) \quad (6064)$$

$$\tau^6_{\gamma,\delta,w,i} = \sum_{\alpha \in B} \tau^5_{\gamma,\alpha,i} \tau^3_{\gamma,\delta,\alpha,w} \quad (2r_D r_T^2 r_V N_o) \quad (6065)$$

$$\tau^7_{\gamma,\delta,w} = \sum_{a \in V} {}^2D^1_{a,w} Y^1_{a,\gamma} Y^{1,*}_{a,\delta} \quad (3r_D r_T^2 N_v) \quad (6066)$$

$${}^2R^z_{\gamma,\delta} \leftarrow \sum_{\epsilon \in A} \sum_{w \in D} \sum_{i \in O} \frac{1}{2} {}^2D^2_{i,w} Y^{2,*}_{i,\gamma} \tau^7_{\epsilon,\gamma,w} \tau^6_{\epsilon,\delta,w,i} \quad (4r_D r_T^3 N_o) \quad (6067)$$

Raw expression

$${}^2R^z_{\epsilon,\zeta} \leftarrow \sum_{i \in O} \sum_{j \in O} \sum_{a \in V} \sum_{b \in V} \sum_{c \in V} \frac{1}{2} Y^{1,*}_{a,\epsilon} Y^{2,*}_{i,\epsilon} Y^{3,*}_{b,\zeta} Y^{4,*}_{j,\zeta} f_{b,c} {}^2D^{a,i,b,j} {}^2T_{c,j,a,i} \quad (6068)$$

Factorized expression

$$\tau^0_{\gamma,\alpha,w} = \sum_{i \in O} {}^2D^4_{i,w} W^4_{i,\alpha} Y^{4,*}_{i,\gamma} \quad (3r_D r_T r_V N_o) \quad (6069)$$

$$\tau^1_{\gamma,\delta,w} = \sum_{a \in V} {}^2D^3_{a,w} Y^1_{a,\gamma} Y^{3,*}_{a,\delta} \quad (3r_D r_T^2 N_v) \quad (6070)$$

$$\tau^3_{\alpha,i} = \sum_{a \in V} {}^1T_{a,i} W^2_{a,\alpha} \quad (2r_V N_o N_v) \quad (6082)$$

$$\tau^2_{\gamma,\delta,w,i} = \sum_{\epsilon \in A} Y^2_{i,\epsilon} Z_{\epsilon,\gamma} \tau^1_{\epsilon,\delta,w} \quad (3r_D r_T^3 N_o) \quad (6071)$$

$$\tau^4_{\gamma,\alpha,w} = \sum_{i \in O} {}^2D^2_{i,w} Y^{2,*}_{i,\gamma} \tau^3_{\alpha,i} \quad (3r_D r_T r_V N_o) \quad (6083)$$

$$\tau^3_{\gamma,\delta,\alpha,w} = \sum_{i \in O} W^3_{i,\alpha} \tau^0_{\delta,\alpha,w} \tau^2_{\gamma,\delta,w,i} \quad (3r_D r_T^2 r_V N_o) \quad (6072)$$

$$\tau^5_{\gamma,w,i} = \sum_{a \in V} {}^2D^1_{a,w} {}^1T_{a,i} Y^{1,*}_{a,\gamma} \quad (3r_D r_T N_o N_v) \quad (6084)$$

$$\tau^4_{\alpha,i,j} = \sum_{\beta \in B} W^1_{i,\beta} W^2_{j,\beta} X_{\beta,\alpha} \quad (3r_V^2 N_o^2) \quad (6073)$$

$$\tau^6_{\gamma,\alpha,w} = \sum_{i \in O} W^1_{i,\alpha} \tau^5_{\gamma,w,i} \quad (2r_D r_T r_V N_o) \quad (6085)$$

$$\tau^5_{\gamma,\alpha,i} = \sum_{j \in O} Y^4_{j,\gamma} \tau^4_{\alpha,j,i} \quad (2r_T r_V N_o^2) \quad (6074)$$

$$\tau^7_{\gamma,\alpha,w} = \sum_{\beta \in B} X_{\beta,\alpha} \tau^4_{\gamma,\beta,w} \tau^6_{\gamma,\beta,w} \quad (3r_D r_T r_V^2) \quad (6086)$$

$$\tau^6_{\gamma,\delta,w,i} = \sum_{\alpha \in B} \tau^5_{\gamma,\alpha,i} \tau^3_{\gamma,\delta,\alpha,w} \quad (2r_D r_T^2 r_V N_o) \quad (6075)$$

$${}^2R^z_{\gamma,\delta} \leftarrow \sum_{\alpha \in B} \sum_{w \in D} \tau^1_{\delta,\alpha,w} \tau^2_{\delta,\alpha,w} \tau^7_{\gamma,\alpha,w} \quad (3r_D r_T^2 r_V) \quad (6087)$$

$$\tau^7_{\gamma,\delta,w} = \sum_{a \in V} {}^2D^1_{a,w} Y^3_{a,\gamma} Y^{1,*}_{a,\delta} \quad (3r_D r_T^2 N_v) \quad (6076)$$

Raw expression

$${}^2R^z_{\gamma,\delta} \leftarrow \sum_{\epsilon \in A} \sum_{w \in D} \sum_{i \in O} \frac{1}{2} {}^2D^2_{i,w} Y^{2,*}_{i,\gamma} \tau^7_{\epsilon,\gamma,w} \tau^6_{\epsilon,\delta,w,i} \quad (4r_D r_T^3 N_o^3) \quad (6077)$$

$$\zeta \leftarrow - \sum_{i \in O} \sum_{j \in O} \sum_{k \in O} \sum_{a \in V} \sum_{b \in V} \sum_{c \in V} \sum_{d \in V} {}^1T_{b,k} {}^1T_{c,i} {}^1T_{d,j} Y^{1,*}_{a,\epsilon} Y^{2,*}_{i,\epsilon} Y^{3,*}_{b,\zeta} Y^{4,*}_{j,\zeta} {}^2D^{a,i,b,j} V_{a,c,k,d} \quad (6088)$$

### E. Contributions from $(H^1 T^1 T^1 T)_c$

Factorized expression

Raw expression

$${}^2R^z_{\epsilon,\zeta} \leftarrow - \sum_{i \in O} \sum_{j \in O} \sum_{k \in O} \sum_{a \in V} \sum_{b \in V} \sum_{c \in V} \sum_{d \in V} {}^1T_{a,k} {}^1T_{c,i} {}^1T_{d,j} Y^{1,*}_{a,\epsilon} Y^{2,*}_{i,\epsilon} Y^{3,*}_{b,\zeta} Y^{4,*}_{j,\zeta} {}^2D^{a,i,b,j} V_{b,d,k,c} \quad (6078)$$

$$\tau^0_{\alpha,i} = \sum_{a \in V} {}^1T_{a,i} W^4_{a,\alpha} \quad (2r_V N_o N_v) \quad (6089)$$

$$\tau^1_{\gamma,\alpha,w} = \sum_{i \in O} {}^2D^4_{i,w} Y^{4,*}_{i,\gamma} \tau^0_{\alpha,i} \quad (3r_D r_T r_V N_o) \quad (6090)$$

Factorized expression

$$\tau^0_{\gamma,w,i} = \sum_{a \in V} {}^2D^3_{a,w} {}^1T_{a,i} Y^{3,*}_{a,\gamma} \quad (3r_D r_T N_o N_v) \quad (6079)$$

$$\tau^2_{\gamma,w,i} = \sum_{a \in V} {}^2D^3_{a,w} {}^1T_{a,i} Y^{3,*}_{a,\gamma} \quad (3r_D r_T N_o N_v) \quad (6091)$$

$$\tau^1_{\gamma,\alpha,w} = \sum_{i \in O} W^3_{i,\alpha} \tau^0_{\gamma,w,i} \quad (2r_D r_T r_V N_o) \quad (6080)$$

$$\tau^3_{\gamma,\alpha,w} = \sum_{i \in O} W^3_{i,\alpha} \tau^2_{\gamma,w,i} \quad (2r_D r_T r_V N_o) \quad (6092)$$

$$\tau^2_{\gamma,\alpha,w} = \sum_{i \in O} {}^2D^4_{i,w} W^4_{i,\alpha} Y^{4,*}_{i,\gamma} \quad (3r_D r_T r_V N_o) \quad (6081)$$

$$\tau^4_{\gamma,w,i} = \sum_{a \in V} {}^2D^1_{a,w} {}^1T_{a,i} Y^{1,*}_{a,\gamma} \quad (3r_D r_T N_o N_v) \quad (6093)$$

$$\tau_{\gamma,\alpha,w}^5 = \sum_{i \in O} W_{i,\alpha}^1 \tau_{\gamma,w,i}^4 \quad (2r_D r_T r_V N_o) \quad (6094)$$

$$\tau_{\gamma,\alpha,w}^6 = \sum_{i \in O} {}^2D_{i,w}^2 W_{i,\alpha}^2 Y_{i,\gamma}^{2,*} \quad (3r_D r_T r_V N_o) \quad (6095)$$

$$\tau_{\gamma,\alpha,w}^7 = \sum_{\beta \in B} X_{\beta,\alpha} \tau_{\gamma,\beta,w}^5 \tau_{\gamma,\beta,w}^6 \quad (3r_D r_T r_V^2) \quad (6096)$$

$${}^2R_{\gamma,\delta}^z \leftarrow \sum_{\alpha \in B} \sum_{w \in D} \tau_{\delta,\alpha,w}^1 \tau_{\delta,\alpha,w}^3 \tau_{\gamma,\alpha,w}^7 \quad (3r_D r_T^2 r_V) \quad (6097)$$

Raw expression

$${}^2R_{\epsilon,\zeta}^z \leftarrow \sum_{i \in O} \sum_{j \in O} \sum_{k \in O} \sum_{l \in O} \sum_{a \in V} \sum_{b \in V} \sum_{c \in V} {}^1T_{a,k} {}^1T_{b,l} {}^1T_{c,i} Y_{a,\epsilon}^{1,*} Y_{i,\epsilon}^{2,*} Y_{b,\zeta}^{3,*} Y_{j,\zeta}^{4,*} {}^2D_{a,i,b,j} V_{k,c,l,j} \quad (6098)$$

Factorized expression

$$\tau_{\alpha,i}^0 = \sum_{a \in V} {}^1T_{a,i} W_{a,\alpha}^2 \quad (2r_V N_o N_v) \quad (6099)$$

$$\tau_{\gamma,\alpha,w}^1 = \sum_{i \in O} {}^2D_{i,w}^4 Y_{i,\gamma}^{4,*} \tau_{\alpha,i}^0 \quad (3r_D r_T r_V N_o) \quad (6100)$$

$$\tau_{\gamma,\alpha,w}^2 = \sum_{a \in V} {}^2D_{a,w}^3 W_{a,\alpha}^1 Y_{a,\gamma}^{3,*} \quad (3r_D r_T r_V N_v) \quad (6101)$$

$$\tau_{\gamma,\alpha,w}^3 = \sum_{\beta \in B} X_{\beta,\alpha} \tau_{\gamma,\beta,w}^1 \tau_{\gamma,\beta,w}^2 \quad (3r_D r_T r_V^2) \quad (6102)$$

$$\tau_{\alpha,i}^4 = \sum_{a \in V} {}^1T_{a,i} W_{a,\alpha}^4 \quad (2r_V N_o N_v) \quad (6103)$$

$$\tau_{\gamma,\alpha,w}^5 = \sum_{i \in O} {}^2D_{i,w}^2 Y_{i,\gamma}^{2,*} \tau_{\alpha,i}^4 \quad (3r_D r_T r_V N_o) \quad (6104)$$

$$\tau_{\gamma,w,i}^6 = \sum_{a \in V} {}^2D_{a,w}^1 {}^1T_{a,i} Y_{a,\gamma}^{1,*} \quad (3r_D r_T N_o N_v) \quad (6105)$$

$$\tau_{\gamma,\alpha,w}^7 = \sum_{i \in O} W_{i,\alpha}^3 \tau_{\gamma,w,i}^6 \quad (2r_D r_T r_V N_o) \quad (6106)$$

$${}^2R_{\gamma,\delta}^z \leftarrow - \sum_{\alpha \in B} \sum_{w \in D} \tau_{\delta,\alpha,w}^3 \tau_{\gamma,\alpha,w}^5 \tau_{\gamma,\alpha,w}^7 \quad (3r_D r_T^2 r_V) \quad (6107)$$

Raw expression

$${}^2R_{\epsilon,\zeta}^z \leftarrow \sum_{i \in O} \sum_{j \in O} \sum_{k \in O} \sum_{l \in O} \sum_{a \in V} \sum_{b \in V} \sum_{c \in V} {}^1T_{a,k} {}^1T_{b,l} {}^1T_{c,j} Y_{a,\epsilon}^{1,*} Y_{i,\epsilon}^{2,*} Y_{b,\zeta}^{3,*} Y_{j,\zeta}^{4,*} {}^2D_{a,i,b,j} V_{k,i,l,c} \quad (6108)$$

Factorized expression

$$\tau_{\alpha,i}^0 = \sum_{a \in V} {}^1T_{a,i} W_{a,\alpha}^4 \quad (2r_V N_o N_v) \quad (6109)$$

$$\tau_{\gamma,\alpha,w}^1 = \sum_{i \in O} {}^2D_{i,w}^4 Y_{i,\gamma}^{4,*} \tau_{\alpha,i}^0 \quad (3r_D r_T r_V N_o) \quad (6110)$$

$$\tau_{\gamma,w,i}^2 = \sum_{a \in V} {}^2D_{a,w}^3 {}^1T_{a,i} Y_{a,\gamma}^{3,*} \quad (3r_D r_T N_o N_v) \quad (6111)$$

$$\tau_{\gamma,\alpha,w}^3 = \sum_{i \in O} W_{i,\alpha}^3 \tau_{\gamma,w,i}^2 \quad (2r_D r_T r_V N_o) \quad (6112)$$

$$\tau_{\alpha,i}^4 = \sum_{a \in V} {}^1T_{a,i} W_{a,\alpha}^2 \quad (2r_V N_o N_v) \quad (6113)$$

$$\tau_{\gamma,\alpha,w}^5 = \sum_{i \in O} {}^2D_{i,w}^2 Y_{i,\gamma}^{2,*} \tau_{\alpha,i}^4 \quad (3r_D r_T r_V N_o) \quad (6114)$$

$$\tau_{\gamma,\alpha,w}^6 = \sum_{a \in V} {}^2D_{a,w}^1 W_{a,\alpha}^1 Y_{a,\gamma}^{1,*} \quad (3r_D r_T r_V N_v) \quad (6115)$$

$$\tau_{\gamma,\alpha,w}^7 = \sum_{\beta \in B} X_{\beta,\alpha} \tau_{\gamma,\beta,w}^5 \tau_{\gamma,\beta,w}^6 \quad (3r_D r_T r_V^2) \quad (6116)$$

$${}^2R_{\gamma,\delta}^z \leftarrow - \sum_{\alpha \in B} \sum_{w \in D} \tau_{\delta,\alpha,w}^1 \tau_{\delta,\alpha,w}^3 \tau_{\gamma,\alpha,w}^7 \quad (3r_D r_T^2 r_V) \quad (6117)$$



### F. Contributions from $(H^1 T^2 T)_c$

Raw expression

$${}^2R^z_{\epsilon,\zeta} \leftarrow - \sum_{i \in O} \sum_{j \in O} \sum_{k \in O} \sum_{a \in V} \sum_{b \in V} \sum_{c \in V} \frac{1}{2} {}^1T_{a,k} {}^Y{}^{1,*}_{a,\epsilon} {}^{Y^2,*}_{i,\epsilon} {}^{Y^3,*}_{b,\zeta} {}^{Y^4,*}_{j,\zeta} f_{k,c} {}^2D^{a,i,b,j} {}^2T_{b,j,c,i} \quad (6118)$$

Factorized expression

$$\tau^0_{\gamma,\delta,w} = \sum_{a \in V} {}^2D^3_{a,w} Y^1_{a,\gamma} Y^{3,*}_{a,\delta} \quad (3r_D r_T^2 N_v) \quad (6119)$$

$$\tau^1_{\gamma,\delta,w} = \sum_{i \in O} {}^2D^4_{i,w} Y^2_{i,\gamma} Y^{4,*}_{i,\delta} \quad (3r_D r_T^2 N_o) \quad (6120)$$

$$\tau^2_{\alpha,i} = \sum_{a \in V} {}^1T_{a,i} W^2_{a,\alpha} \quad (2r_V N_o N_v) \quad (6121)$$

$$\tau^3_{\gamma,\alpha,w} = \sum_{i \in O} {}^2D^2_{i,w} Y^{2,*}_{i,\gamma} \tau^2_{\alpha,i} \quad (3r_D r_T r_V N_o) \quad (6122)$$

$$\tau^4_{\gamma,\alpha,w} = \sum_{a \in V} {}^2D^1_{a,w} W^1_{a,\alpha} Y^{1,*}_{a,\gamma} \quad (3r_D r_T r_V N_v) \quad (6123)$$

$$\tau^5_{\gamma,\alpha} = \sum_{a \in V} W^4_{a,\alpha} Y^3_{a,\gamma} \quad (2r_T r_V N_v) \quad (6124)$$

$$\tau^6_{\gamma,\alpha} = \sum_{i \in O} W^3_{i,\alpha} Y^4_{i,\gamma} \quad (2r_T r_V N_o) \quad (6125)$$

$$\tau^7_{\gamma,\alpha} = \sum_{\beta \in B} X_{\alpha,\beta} \tau^5_{\gamma,\beta} \tau^6_{\gamma,\beta} \quad (3r_T r_V^2) \quad (6126)$$

$$\tau^8_{\gamma,\alpha} = \sum_{\delta \in A} Z_{\gamma,\delta} \tau^7_{\delta,\alpha} \quad (2r_T^2 r_V) \quad (6127)$$

$$\tau^9_{\gamma,\delta,w} = \sum_{\alpha \in B} \tau^8_{\gamma,\alpha} \tau^3_{\delta,\alpha,w} \tau^4_{\delta,\alpha,w} \quad (3r_D r_T^2 r_V) \quad (6128)$$

$${}^2R^z_{\gamma,\delta} \leftarrow \sum_{\epsilon \in A} \sum_{w \in D} \tau^0_{\epsilon,\delta,w} \tau^1_{\epsilon,\delta,w} \tau^9_{\epsilon,\gamma,w} \quad (3r_D r_T^3) \quad (6129)$$

Raw expression

$${}^2R^z_{\epsilon,\zeta} \leftarrow - \sum_{i \in O} \sum_{j \in O} \sum_{k \in O} \sum_{a \in V} \sum_{b \in V} \sum_{c \in V} \frac{1}{2} {}^1T_{a,k} {}^Y{}^{1,*}_{a,\epsilon} {}^{Y^2,*}_{i,\epsilon} {}^{Y^3,*}_{b,\zeta} {}^{Y^4,*}_{j,\zeta} f_{k,c} {}^2D^{a,i,b,j} {}^2T_{c,i,b,j} \quad (6130)$$

Factorized expression

$$\tau^0_{\alpha,i} = \sum_{a \in V} {}^1T_{a,i} W^2_{a,\alpha} \quad (2r_V N_o N_v) \quad (6131)$$

$$\tau^1_{\gamma,\alpha,w} = \sum_{i \in O} {}^2D^2_{i,w} Y^{2,*}_{i,\gamma} \tau^0_{\alpha,i} \quad (3r_D r_T r_V N_o) \quad (6132)$$

$$\tau^2_{\gamma,\alpha,w} = \sum_{a \in V} {}^2D^1_{a,w} W^1_{a,\alpha} Y^{1,*}_{a,\gamma} \quad (3r_D r_T r_V N_v) \quad (6133)$$

$$\tau^3_{\gamma,\alpha} = \sum_{a \in V} W^4_{a,\alpha} Y^1_{a,\gamma} \quad (2r_T r_V N_v) \quad (6134)$$

$$\tau^4_{\gamma,\alpha} = \sum_{i \in O} W^3_{i,\alpha} Y^2_{i,\gamma} \quad (2r_T r_V N_o) \quad (6135)$$

$$\tau^5_{\gamma,\alpha} = \sum_{\beta \in B} X_{\alpha,\beta} \tau^3_{\gamma,\beta} \tau^4_{\gamma,\beta} \quad (3r_T r_V^2) \quad (6136)$$

$$\tau^6_{\gamma,\alpha} = \sum_{\delta \in A} Z_{\delta,\gamma} \tau^5_{\delta,\alpha} \quad (2r_T^2 r_V) \quad (6137)$$

$$\tau^7_{\gamma,\delta,w} = \sum_{\alpha \in B} \tau^6_{\gamma,\alpha} \tau^1_{\delta,\alpha,w} \tau^2_{\delta,\alpha,w} \quad (3r_D r_T^2 r_V) \quad (6138)$$

$$\tau^8_{\gamma,\delta,w} = \sum_{a \in V} {}^2D^3_{a,w} Y^3_{a,\gamma} Y^{3,*}_{a,\delta} \quad (3r_D r_T^2 N_v) \quad (6139)$$

$$\tau^9_{\gamma,\delta,w} = \sum_{i \in O} {}^2D^4_{i,w} Y^4_{i,\gamma} Y^{4,*}_{i,\delta} \quad (3r_D r_T^2 N_o) \quad (6140)$$

$${}^2R^z_{\gamma,\delta} \leftarrow \sum_{\epsilon \in A} \sum_{w \in D} \tau^7_{\epsilon,\gamma,w} \tau^8_{\epsilon,\delta,w} \tau^9_{\epsilon,\delta,w} \quad (3r_D r_T^3) \quad (6141)$$

Raw expression

$${}^2R^z_{\epsilon,\zeta} \leftarrow - \sum_{i \in O} \sum_{j \in O} \sum_{k \in O} \sum_{a \in V} \sum_{b \in V} \sum_{c \in V} \frac{1}{2} {}^1T_{b,k} {}^Y{}^{1,*}_{a,\epsilon} {}^{Y^2,*}_{i,\epsilon} {}^{Y^3,*}_{b,\zeta} {}^{Y^4,*}_{j,\zeta} f_{k,c} {}^2D^{a,i,b,j} {}^2T_{a,i,c,j} \quad (6142)$$

Factorized expression

$$\tau^0_{\alpha,i} = \sum_{a \in V} {}^1T_{a,i} W^2_{a,\alpha} \quad (2r_V N_o N_v) \quad (6143)$$

$$\tau^1_{\gamma,\alpha,w} = \sum_{i \in O} {}^2D^4_{i,w} Y^{4,*}_{i,\gamma} \tau^0_{\alpha,i} \quad (3r_D r_T r_V N_o) \quad (6144)$$

$$\tau^2_{\gamma,\alpha,w} = \sum_{a \in V} {}^2D^3_{a,w} W^1_{a,\alpha} Y^{3,*}_{a,\gamma} \quad (3r_D r_T r_V N_v) \quad (6145)$$

$$\tau^3_{\gamma,\alpha} = \sum_{a \in V} W^4_{a,\alpha} Y^3_{a,\gamma} \quad (2r_T r_V N_v) \quad (6146)$$

$$\tau^4_{\gamma,\alpha} = \sum_{i \in O} W^3_{i,\alpha} Y^4_{i,\gamma} \quad (2r_T r_V N_o) \quad (6147)$$

$$\tau^5_{\gamma,\alpha} = \sum_{\beta \in B} X_{\alpha,\beta} \tau^3_{\gamma,\beta} \tau^4_{\gamma,\beta} \quad (3r_T r_V^2) \quad (6148)$$

$$\tau^6_{\gamma,\alpha} = \sum_{\delta \in A} Z_{\gamma,\delta} \tau^5_{\delta,\alpha} \quad (2r_T^2 r_V) \quad (6149)$$

$$\tau^7_{\gamma,\delta,w} = \sum_{\alpha \in B} \tau^6_{\gamma,\alpha} \tau^1_{\delta,\alpha,w} \tau^2_{\delta,\alpha,w} \quad (3r_D r_T^2 r_V) \quad (6150)$$

$$\tau^8_{\gamma,\delta,w} = \sum_{a \in V} {}^2D^1_{a,w} Y^1_{a,\gamma} Y^{1,*}_{a,\delta} \quad (3r_D r_T^2 N_v) \quad (6151)$$

$$\tau^9_{\gamma,\delta,w} = \sum_{i \in O} {}^2D^2_{i,w} Y^2_{i,\gamma} Y^{2,*}_{i,\delta} \quad (3r_D r_T^2 N_o) \quad (6152)$$

$${}^2R^z_{\gamma,\delta} \leftarrow \sum_{\epsilon \in A} \sum_{w \in D} \tau^7_{\epsilon,\delta,w} \tau^8_{\epsilon,\gamma,w} \tau^9_{\epsilon,\gamma,w} \quad (3r_D r_T^3) \quad (6153)$$

Raw expression

$${}^2R^z_{\epsilon,\zeta} \leftarrow - \sum_{i \in O} \sum_{j \in O} \sum_{k \in O} \sum_{a \in V} \sum_{b \in V} \sum_{c \in V} \frac{1}{2} {}^1T_{b,k} Y^{1,*}_{a,\epsilon} Y^{2,*}_{i,\epsilon} Y^{3,*}_{b,\zeta} Y^{4,*}_{j,\zeta} f_{k,c} {}^2D^{a,i,b,j} {}^2T_{c,j,a,i} \quad (6154)$$

Factorized expression

$$\tau^0_{\alpha,i} = \sum_{a \in V} {}^1T_{a,i} W^2_{a,\alpha} \quad (2r_V N_o N_v) \quad (6155)$$

$$\tau^1_{\gamma,\alpha,w} = \sum_{i \in O} {}^2D^4_{i,w} Y^{4,*}_{i,\gamma} \tau^0_{\alpha,i} \quad (3r_D r_T r_V N_o) \quad (6156)$$

$$\tau^2_{\gamma,\alpha,w} = \sum_{a \in V} {}^2D^3_{a,w} W^1_{a,\alpha} Y^{3,*}_{a,\gamma} \quad (3r_D r_T r_V N_v) \quad (6157)$$

$$\tau^3_{\gamma,\alpha} = \sum_{a \in V} W^4_{a,\alpha} Y^1_{a,\gamma} \quad (2r_T r_V N_v) \quad (6158)$$

$$\tau^4_{\gamma,\alpha} = \sum_{i \in O} W^3_{i,\alpha} Y^2_{i,\gamma} \quad (2r_T r_V N_o) \quad (6159)$$

$$\tau^5_{\gamma,\alpha} = \sum_{\beta \in B} X_{\alpha,\beta} \tau^3_{\gamma,\beta} \tau^4_{\gamma,\beta} \quad (3r_T r_V^2) \quad (6160)$$

$$\tau^6_{\gamma,\alpha} = \sum_{\delta \in A} Z_{\delta,\gamma} \tau^5_{\delta,\alpha} \quad (2r_T^2 r_V) \quad (6161)$$

$$\tau^7_{\gamma,\delta,w} = \sum_{\alpha \in B} \tau^6_{\gamma,\alpha} \tau^1_{\delta,\alpha,w} \tau^2_{\delta,\alpha,w} \quad (3r_D r_T^2 r_V) \quad (6162)$$

$$\tau^8_{\gamma,\delta,w} = \sum_{a \in V} {}^2D^1_{a,w} Y^3_{a,\gamma} Y^{1,*}_{a,\delta} \quad (3r_D r_T^2 N_v) \quad (6163)$$

$$\tau^9_{\gamma,\delta,w} = \sum_{i \in O} {}^2D^2_{i,w} Y^4_{i,\gamma} Y^{2,*}_{i,\delta} \quad (3r_D r_T^2 N_o) \quad (6164)$$

$${}^2R^z_{\gamma,\delta} \leftarrow \sum_{\epsilon \in A} \sum_{w \in D} \tau^7_{\epsilon,\delta,w} \tau^8_{\epsilon,\gamma,w} \tau^9_{\epsilon,\gamma,w} \quad (3r_D r_T^3) \quad (6165)$$

Raw expression

$${}^2R^z_{\epsilon,\zeta} \leftarrow - \sum_{i \in O} \sum_{j \in O} \sum_{k \in O} \sum_{a \in V} \sum_{b \in V} \sum_{c \in V} \frac{1}{2} {}^1T_{c,i} Y^{1,*}_{a,\epsilon} Y^{2,*}_{i,\epsilon} Y^{3,*}_{b,\zeta} Y^{4,*}_{j,\zeta} f_{k,c} {}^2D^{a,i,b,j} {}^2T_{a,k,b,j} \quad (6166)$$

Factorized expression

$$\tau^0_{\gamma,\delta,w} = \sum_{i \in O} {}^2D^2_{i,w} Y^4_{i,\gamma} Y^{2,*}_{i,\delta} \quad (3r_D r_T^2 N_o) \quad (6167)$$

$$\tau^1_{\alpha,i} = \sum_{a \in V} {}^1T_{a,i} W^4_{a,\alpha} \quad (2r_V N_o N_v) \quad (6168)$$

$$\tau^2_{\alpha} = \sum_{i \in O} W^3_{i,\alpha} \tau^1_{\alpha,i} \quad (2r_V N_o) \quad (6169)$$

$$\tau^3_{\alpha} = \sum_{\beta \in B} \tau^2_{\beta} X_{\alpha,\beta} \quad (2r_V^2) \quad (6170)$$

$$\tau^4_{a,b} = \sum_{\alpha \in B} \tau^3_{\alpha} W^1_{a,\alpha} W^2_{b,\alpha} \quad (3r_V N_v^2) \quad (6171)$$

$$\tau^5_{\gamma,a} = \sum_{b \in V} Y^3_{b,\gamma} \tau^4_{a,b} \quad (2r_T N_v^2) \quad (6172)$$

$$\tau^6_{\gamma,\delta,w} = \sum_{a \in V} {}^2D^1_{a,w} Y^{1,*}_{a,\delta} \tau^5_{\gamma,a} \quad (3r_D r_T^2 N_v) \quad (6173)$$

$$\tau^7_{\gamma,\delta,w} = \sum_{\epsilon \in A} Z_{\gamma,\epsilon} \tau^0_{\epsilon,\delta,w} \tau^6_{\epsilon,\delta,w} \quad (3r_D r_T^3) \quad (6174)$$

$$\tau^8_{\gamma,\delta,w} = \sum_{a \in V} {}^2D^3_{a,w} Y^1_{a,\gamma} Y^{3,*}_{a,\delta} \quad (3r_D r_T^2 N_v) \quad (6175)$$

$$\tau^9_{\gamma,\delta,w} = \sum_{i \in O} {}^2D^4_{i,w} Y^2_{i,\gamma} Y^{4,*}_{i,\delta} \quad (3r_D r_T^2 N_o) \quad (6176)$$

$${}^2R^z_{\gamma,\delta} \leftarrow \sum_{\epsilon \in A} \sum_{w \in D} \tau^7_{\epsilon,\gamma,w} \tau^8_{\epsilon,\delta,w} \tau^9_{\epsilon,\delta,w} \quad (3r_D r_T^3) \quad (6177)$$

Raw expression

$${}^2R^z_{\epsilon,\zeta} \leftarrow - \sum_{i \in O} \sum_{j \in O} \sum_{k \in O} \sum_{a \in V} \sum_{b \in V} \sum_{c \in V} \frac{1}{2} {}^1T_{c,i} Y^{1,*}_{a,\epsilon} Y^{2,*}_{i,\epsilon} Y^{3,*}_{b,\zeta} Y^{4,*}_{j,\zeta} f_{k,c} {}^2D^{a,i,b,j} {}^2T_{b,j,a,k} \quad (6178)$$

Factorized expression

$$\tau^0_{\gamma,\delta,w} = \sum_{i \in O} {}^2D^2_{i,w} Y^2_{i,\gamma} Y^{2,*}_{i,\delta} \quad (3r_D r_T^2 N_o) \quad (6179)$$

$$\tau^1_{\alpha,i} = \sum_{a \in V} {}^1T_{a,i} W^4_{a,\alpha} \quad (2r_V N_o N_v) \quad (6180)$$

$$\tau^2_{\alpha} = \sum_{i \in O} W^3_{i,\alpha} \tau^1_{\alpha,i} \quad (2r_V N_o) \quad (6181)$$

$$\tau^3_{\alpha} = \sum_{\beta \in B} \tau^2_{\beta} X_{\alpha,\beta} \quad (2r_V^2) \quad (6182)$$

$$\tau^4_{a,b} = \sum_{\alpha \in B} \tau^3_{\alpha} W^1_{a,\alpha} W^2_{b,\alpha} \quad (3r_V N_v^2) \quad (6183)$$

$$\tau^5_{\gamma,a} = \sum_{b \in V} Y^1_{b,\gamma} \tau^4_{a,b} \quad (2r_T N_v^2) \quad (6184)$$

$$\tau^6_{\gamma,\delta,w} = \sum_{a \in V} {}^2D^1_{a,w} Y^{1,*}_{a,\delta} \tau^5_{\gamma,a} \quad (3r_D r_T^2 N_v) \quad (6185)$$

$$\tau^7_{\gamma,\delta,w} = \sum_{a \in V} {}^2D^3_{a,w} Y^3_{a,\gamma} Y^{3,*}_{a,\delta} \quad (3r_D r_T^2 N_v) \quad (6186)$$

$$\tau^8_{\gamma,\delta,w} = \sum_{i \in O} {}^2D^4_{i,w} Y^4_{i,\gamma} Y^{4,*}_{i,\delta} \quad (3r_D r_T^2 N_o) \quad (6187)$$

$$\tau^9_{\gamma,\delta,w} = \sum_{\epsilon \in A} Z_{\gamma,\epsilon} \tau^7_{\epsilon,\delta,w} \tau^8_{\epsilon,\delta,w} \quad (3r_D r_T^3) \quad (6188)$$

$${}^2R^z_{\gamma,\delta} \leftarrow \sum_{\epsilon \in A} \sum_{w \in D} \tau^0_{\epsilon,\gamma,w} \tau^6_{\epsilon,\gamma,w} \tau^9_{\epsilon,\delta,w} \quad (3r_D r_T^3) \quad (6189)$$

Raw expression

$${}^2R^z_{\epsilon,\zeta} \leftarrow - \sum_{i \in O} \sum_{j \in O} \sum_{k \in O} \sum_{a \in V} \sum_{b \in V} \sum_{c \in V} \frac{1}{2} {}^1T_{c,j} Y^{1,*}_{a,\epsilon} Y^{2,*}_{i,\epsilon} Y^{3,*}_{b,\zeta} Y^{4,*}_{j,\zeta} f_{k,c} {}^2D^{a,i,b,j} {}^2T_{a,i,b,k} \quad (6190)$$

Factorized expression

$$\tau^0_{\gamma,\delta,w} = \sum_{a \in V} {}^2D^1_{a,w} Y^1_{a,\gamma} Y^{1,*}_{a,\delta} \quad (3r_D r_T^2 N_v) \quad (6191)$$

$$\tau^1_{\gamma,\delta,w} = \sum_{i \in O} {}^2D^2_{i,w} Y^2_{i,\gamma} Y^{2,*}_{i,\delta} \quad (3r_D r_T^2 N_o) \quad (6192)$$

$$\tau^2_{\gamma,\delta,w} = \sum_{i \in O} {}^2D^4_{i,w} Y^4_{i,\gamma} Y^{4,*}_{i,\delta} \quad (3r_D r_T^2 N_o) \quad (6193)$$

$$\tau^3_{\alpha,i} = \sum_{a \in V} {}^1T_{a,i} W^4_{a,\alpha} \quad (2r_V N_o N_v) \quad (6194)$$

$$\tau^4_{\alpha} = \sum_{i \in O} W^3_{i,\alpha} \tau^3_{\alpha,i} \quad (2r_V N_o) \quad (6195)$$

$$\tau^5_{\alpha} = \sum_{\beta \in B} \tau^4_{\beta} X_{\alpha,\beta} \quad (2r_V{}^2) \quad (6196)$$

$$\tau^6_{a,b} = \sum_{\alpha \in B} \tau^5_{\alpha} W^1_{a,\alpha} W^2_{b,\alpha} \quad (3r_V N_v{}^2) \quad (6197)$$

$$\tau^7_{\gamma,a} = \sum_{b \in V} Y^3_{b,\gamma} \tau^6_{a,b} \quad (2r_T N_v{}^2) \quad (6198)$$

$$\tau^8_{\gamma,\delta,w} = \sum_{a \in V} {}^2D^3_{a,w} Y^{3,*}_{a,\delta} \tau^7_{\gamma,a} \quad (3r_D r_T{}^2 N_v) \quad (6199)$$

$$\tau^9_{\gamma,\delta,w} = \sum_{\epsilon \in A} Z_{\gamma,\epsilon} \tau^2_{\epsilon,\delta,w} \tau^8_{\epsilon,\delta,w} \quad (3r_D r_T{}^3) \quad (6200)$$

$${}^2R^z_{\gamma,\delta} \leftarrow \sum_{\epsilon \in A} \sum_{w \in D} \tau^0_{\epsilon,\gamma,w} \tau^1_{\epsilon,\gamma,w} \tau^9_{\epsilon,\delta,w} \quad (3r_D r_T{}^3) \quad (6201)$$

Raw expression

$${}^2R^z_{\epsilon,\zeta} \leftarrow - \sum_{i \in O} \sum_{j \in O} \sum_{k \in O} \sum_{a \in V} \sum_{b \in V} \sum_{c \in V} \frac{1}{2} {}^1T_{c,j} Y^{1,*}_{a,\epsilon} Y^{2,*}_{i,\epsilon} Y^{3,*}_{b,\zeta} Y^{4,*}_{j,\zeta} f_{k,c} {}^2D^{a,i,b,j} {}^2T_{b,k,a,i} \quad (6202)$$

Factorized expression

$$\tau^0_{\gamma,\delta,w} = \sum_{a \in V} {}^2D^1_{a,w} Y^3_{a,\gamma} Y^{1,*}_{a,\delta} \quad (3r_D r_T{}^2 N_v) \quad (6203)$$

$$\tau^1_{\gamma,\delta,w} = \sum_{i \in O} {}^2D^2_{i,w} Y^4_{i,\gamma} Y^{2,*}_{i,\delta} \quad (3r_D r_T{}^2 N_o) \quad (6204)$$

$$\tau^2_{\gamma,\delta,w} = \sum_{\epsilon \in A} Z_{\gamma,\epsilon} \tau^0_{\epsilon,\delta,w} \tau^1_{\epsilon,\delta,w} \quad (3r_D r_T{}^3) \quad (6205)$$

$$\tau^3_{\gamma,\delta,w} = \sum_{i \in O} {}^2D^4_{i,w} Y^2_{i,\gamma} Y^{4,*}_{i,\delta} \quad (3r_D r_T{}^2 N_o) \quad (6206)$$

$$\tau^4_{\alpha,i} = \sum_{a \in V} {}^1T_{a,i} W^4_{a,\alpha} \quad (2r_V N_o N_v) \quad (6207)$$

$$\tau^5_{\alpha} = \sum_{i \in O} W^3_{i,\alpha} \tau^4_{\alpha,i} \quad (2r_V N_o) \quad (6208)$$

$$\tau^6_{\alpha} = \sum_{\beta \in B} \tau^5_{\beta} X_{\alpha,\beta} \quad (2r_V{}^2) \quad (6209)$$

$$\tau^7_{a,b} = \sum_{\alpha \in B} \tau^6_{\alpha} W^1_{a,\alpha} W^2_{b,\alpha} \quad (3r_V N_v{}^2) \quad (6210)$$

$$\tau^8_{\gamma,a} = \sum_{b \in V} Y^1_{b,\gamma} \tau^7_{a,b} \quad (2r_T N_v{}^2) \quad (6211)$$

$$\tau^9_{\gamma,\delta,w} = \sum_{a \in V} {}^2D^3_{a,w} Y^{3,*}_{a,\delta} \tau^8_{\gamma,a} \quad (3r_D r_T{}^2 N_v) \quad (6212)$$

$${}^2R^z_{\gamma,\delta} \leftarrow \sum_{\epsilon \in A} \sum_{w \in D} \tau^2_{\epsilon,\gamma,w} \tau^3_{\epsilon,\delta,w} \tau^9_{\epsilon,\delta,w} \quad (3r_D r_T{}^3) \quad (6213)$$

Raw expression

$${}^2R^z_{\epsilon,\zeta} \leftarrow \sum_{i \in O} \sum_{j \in O} \sum_{k \in O} \sum_{a \in V} \sum_{b \in V} \sum_{c \in V} \sum_{d \in V} {}^1T_{c,i} Y^{1,*}_{a,\epsilon} Y^{2,*}_{i,\epsilon} Y^{3,*}_{b,\zeta} Y^{4,*}_{j,\zeta} {}^2D^{a,i,b,j} {}^2T_{b,j,d,k} V_{a,c,k,d} \quad (6214)$$

Factorized expression

$$\tau^0_{\gamma,w,i} = \sum_{a \in V} {}^2D^1_{a,w} {}^1T_{a,i} Y^{1,*}_{a,\gamma} \quad (3r_D r_T N_o N_v) \quad (6215)$$

$$\tau^1_{\gamma,\alpha,w} = \sum_{a \in V} {}^2D^3_{a,w} W^1_{a,\alpha} Y^{3,*}_{a,\gamma} \quad (3r_D r_T r_V N_v) \quad (6216)$$

$$\tau^2_{\gamma,\alpha} = \sum_{a \in V} W^2_{a,\alpha} Y^1_{a,\gamma} \quad (2r_T r_V N_v) \quad (6217)$$

$$\tau^3_{\gamma,\alpha,i} = \sum_{\delta \in A} Y^2_{i,\delta} Z_{\delta,\gamma} \tau^2_{\delta,\alpha} \quad (3r_T{}^2 r_V N_o) \quad (6218)$$

$$\tau^4_{\gamma,\delta,\alpha,w} = \sum_{i \in O} {}^2D^4_{i,w} Y^{4,*}_{i,\delta} \tau^1_{\delta,\alpha,w} \tau^3_{\gamma,\alpha,i} \quad (4r_D r_T{}^2 r_V N_o) \quad (6219)$$

$$\tau^5_{\gamma,\alpha} = \sum_{a \in V} W^4_{a,\alpha} Y^3_{a,\gamma} \quad (2r_T r_V N_v) \quad (6220)$$

$$\tau_{\gamma,\alpha,i}^6 = \sum_{\beta \in B} X_{\alpha,\beta} W_{i,\beta}^3 \tau_{\gamma,\beta}^5 \quad (3r_T r_V^2 N_o) \quad (6221)$$

$$\tau_{\gamma,\delta,w,i}^7 = \sum_{\alpha \in B} \tau_{\gamma,\alpha,i}^6 \tau_{\gamma,\delta,\alpha,w}^4 \quad (2r_D r_T^2 r_V N_o) \quad (6233)$$

$$\tau_{\gamma,\delta,w,i}^7 = \sum_{\alpha \in B} \tau_{\gamma,\alpha,i}^6 \tau_{\gamma,\delta,\alpha,w}^4 \quad (2r_D r_T^2 r_V N_o) \quad (6222)$$

$$\tau_{\gamma,w,i,j}^8 = \sum_{\delta \in A} Y_{j,\delta}^2 \tau_{\delta,\gamma,w,i}^7 \quad (2r_D r_T^2 N_o^2) \quad (6234)$$

$$\tau_{\gamma,w,i,j}^8 = \sum_{\delta \in A} Y_{j,\delta}^4 \tau_{\delta,\gamma,w,i}^7 \quad (2r_D r_T^2 N_o^2) \quad (6223)$$

$${}^2R_{\gamma,\delta}^z \leftarrow - \sum_{w \in D} \sum_{i \in O} \sum_{j \in O} \frac{1}{2} {}^2D_{i,w}^2 Y_{i,\gamma}^{2,*} \tau_{\gamma,w,j}^0 \tau_{\delta,w,j,i}^8 \quad (4r_D r_T^2 N_o^2) \quad (6235)$$

$${}^2R_{\gamma,\delta}^z \leftarrow - \sum_{w \in D} \sum_{i \in O} \sum_{j \in O} \frac{1}{2} {}^2D_{i,w}^2 Y_{i,\gamma}^{2,*} \tau_{\gamma,w,j}^0 \tau_{\delta,w,j,i}^8 \quad (4r_D r_T^2 N_o^2) \quad (6224)$$

Raw expression

$${}^2R_{\epsilon,\zeta}^z \leftarrow \sum_{i \in O} \sum_{j \in O} \sum_{k \in O} \sum_{a \in V} \sum_{b \in V} \sum_{c \in V} \sum_{d \in V} {}^1T_{c,i} Y_{a,\epsilon}^{1,*} Y_{i,\epsilon}^{2,*} Y_{b,\zeta}^{3,*} Y_{j,\zeta}^{4,*} {}^2D_{a,i,b,j} {}^2T_{d,k,b,j} V_{a,c,k,d} \quad (6225)$$

Factorized expression

$$\tau_{\gamma,w,i}^0 = \sum_{a \in V} {}^2D_{a,w}^1 {}^1T_{a,i} Y_{a,\gamma}^{1,*} \quad (3r_D r_T N_o N_v) \quad (6226)$$

$${}^2R_{\epsilon,\zeta}^z \leftarrow \sum_{i \in O} \sum_{j \in O} \sum_{k \in O} \sum_{a \in V} \sum_{b \in V} \sum_{c \in V} \sum_{d \in V} {}^1T_{c,j} Y_{a,\epsilon}^{1,*} Y_{i,\epsilon}^{2,*} Y_{b,\zeta}^{3,*} Y_{j,\zeta}^{4,*} {}^2D_{a,i,b,j} {}^2T_{a,i,d,k} V_{b,c,k,d} \quad (6236)$$

Factorized expression

$$\tau_{\gamma,w,i}^0 = \sum_{a \in V} {}^2D_{a,w}^3 {}^1T_{a,i} Y_{a,\gamma}^{3,*} \quad (3r_D r_T N_o N_v) \quad (6237)$$

$$\tau_{\gamma,\alpha,w}^1 = \sum_{a \in V} {}^2D_{a,w}^1 W_{a,\alpha}^1 Y_{a,\gamma}^{1,*} \quad (3r_D r_T r_V N_v) \quad (6238)$$

$$\tau_{\gamma,\alpha,w}^1 = \sum_{a \in V} {}^2D_{a,w}^3 W_{a,\alpha}^1 Y_{a,\gamma}^{3,*} \quad (3r_D r_T r_V N_v) \quad (6227)$$

$$\tau_{\gamma,\alpha}^2 = \sum_{a \in V} W_{a,\alpha}^2 Y_{a,\gamma}^1 \quad (2r_T r_V N_v) \quad (6239)$$

$$\tau_{\gamma,\alpha}^2 = \sum_{a \in V} W_{a,\alpha}^2 Y_{a,\gamma}^3 \quad (2r_T r_V N_v) \quad (6228)$$

$$\tau_{\gamma,\alpha,i}^3 = \sum_{\delta \in A} Y_{i,\delta}^2 Z_{\delta,\gamma} \tau_{\delta,\alpha}^2 \quad (3r_T^2 r_V N_o) \quad (6240)$$

$$\tau_{\gamma,\alpha,i}^3 = \sum_{\delta \in A} Z_{\gamma,\delta} Y_{i,\delta}^4 \tau_{\delta,\alpha}^2 \quad (3r_T^2 r_V N_o) \quad (6229)$$

$$\tau_{\gamma,\delta,\alpha,w}^4 = \sum_{i \in O} {}^2D_{i,w}^2 Y_{i,\delta}^{2,*} \tau_{\delta,\alpha,w}^1 \tau_{\gamma,\alpha,i}^3 \quad (4r_D r_T^2 r_V N_o) \quad (6241)$$

$$\tau_{\gamma,\delta,\alpha,w}^4 = \sum_{i \in O} {}^2D_{i,w}^4 Y_{i,\delta}^{4,*} \tau_{\delta,\alpha,w}^1 \tau_{\gamma,\alpha,i}^3 \quad (4r_D r_T^2 r_V N_o) \quad (6230)$$

$$\tau_{\gamma,\alpha}^5 = \sum_{a \in V} W_{a,\alpha}^4 Y_{a,\gamma}^3 \quad (2r_T r_V N_v) \quad (6242)$$

$$\tau_{\gamma,\alpha}^5 = \sum_{a \in V} W_{a,\alpha}^4 Y_{a,\gamma}^1 \quad (2r_T r_V N_v) \quad (6231)$$

$$\tau_{\gamma,\alpha,i}^6 = \sum_{\beta \in B} X_{\alpha,\beta} W_{i,\beta}^3 \tau_{\gamma,\beta}^5 \quad (3r_T r_V^2 N_o) \quad (6243)$$

$$\tau_{\gamma,\alpha,i}^6 = \sum_{\beta \in B} X_{\alpha,\beta} W_{i,\beta}^3 \tau_{\gamma,\beta}^5 \quad (3r_T r_V^2 N_o) \quad (6232)$$

$$\tau_{\gamma,\delta,w,i}^7 = \sum_{\alpha \in B} \tau_{\gamma,\alpha,i}^6 \tau_{\gamma,\delta,\alpha,w}^4 \quad (2r_D r_T^2 r_V N_o) \quad (6244)$$

$$\tau_{\gamma,w,i,j}^8 = \sum_{\delta \in A} Y_{j,\delta}^4 \tau_{\delta,\gamma,w,i}^7 \quad (2r_D r_T^2 N_o^2) \quad (6245)$$

$${}^2R_{\gamma,\delta}^z \leftarrow - \sum_{w \in D} \sum_{i \in O} \sum_{j \in O} \frac{1}{2} {}^2D_{i,w}^4 Y_{i,\delta}^{4,*} \tau_{\delta,w,j}^0 \tau_{\gamma,w,j,i}^8 \quad (4r_D r_T^2 N_o^2) \quad (6257)$$

$${}^2R_{\gamma,\delta}^z \leftarrow - \sum_{w \in D} \sum_{i \in O} \sum_{j \in O} \frac{1}{2} {}^2D_{i,w}^4 Y_{i,\delta}^{4,*} \tau_{\delta,w,j}^0 \tau_{\gamma,w,j,i}^8 \quad (4r_D r_T^2 N_o^2) \quad (6246)$$

Raw expression

$${}^2R_{\epsilon,\zeta}^z \leftarrow \sum_{i \in O} \sum_{j \in O} \sum_{k \in O} \sum_{a \in V} \sum_{b \in V} \sum_{c \in V} \sum_{d \in V} {}^1T_{c,k} Y_{a,\epsilon}^{1,*} Y_{i,\epsilon}^{2,*} Y_{b,\zeta}^{3,*} Y_{j,\zeta}^{4,*} {}^2D_{a,i,b,j} {}^2T_{a,i,d,j} V_{b,d,k,c} \quad (6258)$$

$${}^2R_{\epsilon,\zeta}^z \leftarrow \sum_{i \in O} \sum_{j \in O} \sum_{k \in O} \sum_{a \in V} \sum_{b \in V} \sum_{c \in V} \sum_{d \in V} {}^1T_{c,j} Y_{a,\epsilon}^{1,*} Y_{i,\epsilon}^{2,*} Y_{b,\zeta}^{3,*} Y_{j,\zeta}^{4,*} {}^2D_{a,i,b,j} {}^2T_{d,k,a,i} V_{b,c,k,d} \quad (6247)$$

Factorized expression

$$\tau_{\alpha,i}^0 = \sum_{a \in V} {}^1T_{a,i} W_{a,\alpha}^2 \quad (2r_V N_o N_v) \quad (6259)$$

Factorized expression

$$\tau_{\gamma,w,i}^0 = \sum_{a \in V} {}^2D_{a,w}^3 {}^1T_{a,i} Y_{a,\gamma}^{3,*} \quad (3r_D r_T N_o N_v) \quad (6248)$$

$$\tau_{\gamma,\alpha,w}^1 = \sum_{i \in O} {}^2D_{i,w}^2 Y_{i,\gamma}^{2,*} \tau_{\alpha,i}^0 \quad (3r_D r_T r_V N_o) \quad (6260)$$

$$\tau_{\gamma,\alpha,w}^1 = \sum_{a \in V} {}^2D_{a,w}^1 W_{a,\alpha}^1 Y_{a,\gamma}^{1,*} \quad (3r_D r_T r_V N_v) \quad (6249)$$

$$\tau_{\gamma,\alpha,w}^2 = \sum_{a \in V} {}^2D_{a,w}^1 W_{a,\alpha}^1 Y_{a,\gamma}^{1,*} \quad (3r_D r_T r_V N_v) \quad (6261)$$

$$\tau_{\gamma,\alpha}^2 = \sum_{a \in V} W_{a,\alpha}^2 Y_{a,\gamma}^3 \quad (2r_T r_V N_v) \quad (6250)$$

$$\tau_{\gamma,\delta,w}^3 = \sum_{a \in V} {}^2D_{a,w}^3 Y_{a,\gamma}^1 Y_{a,\delta}^{3,*} \quad (3r_D r_T^2 N_v) \quad (6262)$$

$$\tau_{\gamma,\alpha,i}^3 = \sum_{\delta \in A} Z_{\gamma,\delta} Y_{i,\delta}^4 \tau_{\delta,\alpha}^2 \quad (3r_T^2 r_V N_o) \quad (6251)$$

$$\tau_{\gamma,\alpha}^4 = \sum_{i \in O} W_{i,\alpha}^3 Y_{i,\gamma}^2 \quad (2r_T r_V N_o) \quad (6263)$$

$$\tau_{\gamma,\delta,\alpha,w}^4 = \sum_{i \in O} {}^2D_{i,w}^2 Y_{i,\delta}^{2,*} \tau_{\delta,\alpha,w}^1 \tau_{\gamma,\alpha,i}^3 \quad (4r_D r_T^2 r_V N_o) \quad (6252)$$

$$\tau_{\gamma,\alpha}^5 = \sum_{a \in V} W_{a,\alpha}^4 Y_{a,\gamma}^3 \quad (2r_T r_V N_v) \quad (6264)$$

$$\tau_{\gamma,\alpha,i}^6 = \sum_{\delta \in A} Z_{\gamma,\delta} Y_{i,\delta}^4 \tau_{\delta,\alpha}^5 \quad (3r_T^2 r_V N_o) \quad (6265)$$

$$\tau_{\gamma,\alpha}^5 = \sum_{a \in V} W_{a,\alpha}^4 Y_{a,\gamma}^1 \quad (2r_T r_V N_v) \quad (6253)$$

$$\tau_{\gamma,\alpha,w}^7 = \sum_{\delta \in A} \sum_{i \in O} {}^2D_{i,w}^4 Y_{i,\gamma}^{4,*} \tau_{\delta,\alpha}^4 \tau_{\delta,\gamma,w}^3 \tau_{\delta,\alpha,i}^6 \quad (5r_D r_T^2 r_V N_o) \quad (6266)$$

$$\tau_{\gamma,\alpha,i}^6 = \sum_{\beta \in B} X_{\alpha,\beta} W_{i,\beta}^3 \tau_{\gamma,\beta}^5 \quad (3r_T r_V^2 N_o) \quad (6254)$$

$$\tau_{\gamma,\alpha,w}^8 = \sum_{\beta \in B} X_{\alpha,\beta} \tau_{\gamma,\beta,w}^7 \quad (2r_D r_T r_V^2) \quad (6267)$$

$$\tau_{\gamma,\delta,w,i}^7 = \sum_{\alpha \in B} \tau_{\gamma,\alpha,i}^6 \tau_{\gamma,\delta,\alpha,w}^4 \quad (2r_D r_T^2 r_V N_o) \quad (6255)$$

$${}^2R_{\gamma,\delta}^z \leftarrow - \sum_{\alpha \in B} \sum_{w \in D} \frac{1}{2} \tau_{\gamma,\alpha,w}^1 \tau_{\gamma,\alpha,w}^2 \tau_{\delta,\alpha,w}^8 \quad (3r_D r_T^2 r_V) \quad (6268)$$

$$\tau_{\gamma,w,i,j}^8 = \sum_{\delta \in A} Y_{j,\delta}^2 \tau_{\delta,\gamma,w,i}^7 \quad (2r_D r_T^2 N_o^2) \quad (6256)$$

Raw expression

$${}^2R^z_{\epsilon,\zeta} \leftarrow \sum_{i \in O} \sum_{j \in O} \sum_{k \in O} \sum_{a \in V} \sum_{b \in V} \sum_{c \in V} \sum_{d \in V} {}^1T_{c,k} Y^{1,*}_{a,\epsilon} Y^{2,*}_{i,\epsilon} Y^{3,*}_{b,\zeta} Y^{4,*}_{j,\zeta} {}^2D^{a,i,b,j} {}^2T_{b,j,d,i} V_{a,d,k,c} \quad (6269)$$

Factorized expression

$$\tau^0_{\alpha,i} = \sum_{a \in V} {}^1T_{a,i} W^2_{a,\alpha} \quad (2r_V N_o N_v) \quad (6270)$$

$$\tau^1_{\gamma,\alpha,w} = \sum_{i \in O} {}^2D^2_{i,w} Y^{2,*}_{i,\gamma} \tau^0_{\alpha,i} \quad (3r_D r_T r_V N_o) \quad (6271)$$

$$\tau^2_{\gamma,\alpha,w} = \sum_{a \in V} {}^2D^1_{a,w} W^1_{a,\alpha} Y^{1,*}_{a,\gamma} \quad (3r_D r_T r_V N_v) \quad (6272)$$

$$\tau^3_{\gamma,\delta,w} = \sum_{a \in V} {}^2D^3_{a,w} Y^3_{a,\gamma} Y^{3,*}_{a,\delta} \quad (3r_D r_T^2 N_v) \quad (6273)$$

$$\tau^4_{\gamma,\alpha} = \sum_{a \in V} W^4_{a,\alpha} Y^1_{a,\gamma} \quad (2r_T r_V N_v) \quad (6274)$$

$$\tau^5_{\gamma,\alpha,i} = \sum_{\delta \in A} Y^2_{i,\delta} Z_{\delta,\gamma} \tau^4_{\delta,\alpha} \quad (3r_T^2 r_V N_o) \quad (6275)$$

$$\tau^6_{\gamma,\alpha} = \sum_{i \in O} W^3_{i,\alpha} Y^4_{i,\gamma} \quad (2r_T r_V N_o) \quad (6276)$$

$$\tau^7_{\gamma,\alpha,w} = \sum_{\delta \in A} \sum_{i \in O} {}^2D^4_{i,w} Y^{4,*}_{i,\gamma} \tau^6_{\delta,\alpha} \tau^3_{\delta,\gamma,w} \tau^5_{\delta,\alpha,i} \quad (5r_D r_T^2 r_V N_o) \quad (6277)$$

$$\tau^8_{\gamma,\alpha,w} = \sum_{\beta \in B} X_{\alpha,\beta} \tau^7_{\gamma,\beta,w} \quad (2r_D r_T r_V^2) \quad (6278)$$

$${}^2R^z_{\gamma,\delta} \leftarrow - \sum_{\alpha \in B} \sum_{w \in D} \frac{1}{2} \tau^1_{\gamma,\alpha,w} \tau^2_{\gamma,\alpha,w} \tau^8_{\delta,\alpha,w} \quad (3r_D r_T^2 r_V) \quad (6279)$$

Raw expression

$${}^2R^z_{\epsilon,\zeta} \leftarrow \sum_{i \in O} \sum_{j \in O} \sum_{k \in O} \sum_{a \in V} \sum_{b \in V} \sum_{c \in V} \sum_{d \in V} {}^1T_{c,k} Y^{1,*}_{a,\epsilon} Y^{2,*}_{i,\epsilon} Y^{3,*}_{b,\zeta} Y^{4,*}_{j,\zeta} {}^2D^{a,i,b,j} {}^2T_{d,i,b,j} V_{a,d,k,c} \quad (6280)$$

Factorized expression

$$\tau^0_{\alpha,i} = \sum_{a \in V} {}^1T_{a,i} W^4_{a,\alpha} \quad (2r_V N_o N_v) \quad (6281)$$

$$\tau^1_{\alpha,i,j} = \sum_{\beta \in B} X_{\alpha,\beta} W^3_{j,\beta} \tau^0_{\beta,i} \quad (3r_V^2 N_o^2) \quad (6282)$$

$$\tau^2_{\gamma,\alpha,i} = \sum_{j \in O} Y^4_{j,\gamma} \tau^1_{\alpha,i,j} \quad (2r_T r_V N_o^2) \quad (6283)$$

$$\tau^3_{\gamma,\alpha} = \sum_{a \in V} W^2_{a,\alpha} Y^3_{a,\gamma} \quad (2r_T r_V N_v) \quad (6284)$$

$$\tau^4_{\gamma,i,a} = \sum_{\alpha \in B} W^1_{a,\alpha} \tau^3_{\gamma,\alpha} \tau^2_{\gamma,\alpha,i} \quad (3r_T r_V N_o N_v) \quad (6285)$$

$$\tau^5_{\gamma,\delta,w} = \sum_{i \in O} \sum_{a \in V} {}^2D^1_{a,w} {}^2D^2_{i,w} Y^{1,*}_{a,\delta} Y^{2,*}_{i,\delta} \tau^4_{\gamma,i,a} \quad (5r_D r_T^2 N_o N_v) \quad (6286)$$

$$\tau^6_{\gamma,\delta,w} = \sum_{\epsilon \in A} Z_{\gamma,\epsilon} \tau^5_{\epsilon,\delta,w} \quad (2r_D r_T^3) \quad (6287)$$

$$\tau^7_{\gamma,\delta,w} = \sum_{a \in V} {}^2D^3_{a,w} Y^1_{a,\gamma} Y^{3,*}_{a,\delta} \quad (3r_D r_T^2 N_v) \quad (6288)$$

$$\tau^8_{\gamma,\delta,w} = \sum_{i \in O} {}^2D^4_{i,w} Y^2_{i,\gamma} Y^{4,*}_{i,\delta} \quad (3r_D r_T^2 N_o) \quad (6289)$$

$${}^2R^z_{\gamma,\delta} \leftarrow - \sum_{\epsilon \in A} \sum_{w \in D} \frac{1}{2} \tau^6_{\epsilon,\gamma,w} \tau^7_{\epsilon,\delta,w} \tau^8_{\epsilon,\delta,w} \quad (3r_D r_T^3) \quad (6290)$$

Raw expression

$${}^2R^z_{\epsilon,\zeta} \leftarrow \sum_{i \in O} \sum_{j \in O} \sum_{k \in O} \sum_{a \in V} \sum_{b \in V} \sum_{c \in V} \sum_{d \in V} {}^1T_{c,k} Y^{1,*}_{a,\epsilon} Y^{2,*}_{i,\epsilon} Y^{3,*}_{b,\zeta} Y^{4,*}_{j,\zeta} {}^2D^{a,i,b,j} {}^2T_{d,j,a,i} V_{b,d,k,c} \quad (6291)$$

Factorized expression

$$\tau^0_{\alpha,i} = \sum_{a \in V} {}^1T_{a,i} W^4_{a,\alpha} \quad (2r_V N_o N_v) \quad (6292)$$

$$\tau^1_{\alpha,i,j} = \sum_{\beta \in B} X_{\alpha,\beta} W^3_{j,\beta} \tau^0_{\beta,i} \quad (3r_V^2 N_o^2) \quad (6293)$$

$$\tau^2_{\gamma,\alpha,i} = \sum_{j \in O} Y^2_{j,\gamma} \tau^1_{\alpha,i,j} \quad (2r_T r_V N_o^2) \quad (6294)$$

$$\tau^3_{\gamma,\alpha} = \sum_{a \in V} W^2_{a,\alpha} Y^1_{a,\gamma} \quad (2r_T r_V N_v) \quad (6295)$$

$$\tau^4_{\gamma,i,a} = \sum_{\alpha \in B} W^1_{a,\alpha} \tau^3_{\gamma,\alpha} \tau^2_{\gamma,\alpha,i} \quad (3r_T r_V N_o N_v) \quad (6296)$$

$$\tau^5_{\gamma,\delta,w} = \sum_{i \in O} \sum_{a \in V} {}^2D^1_{a,w} {}^2D^2_{i,w} Y^{1,*}_{a,\delta} Y^{2,*}_{i,\delta} \tau^4_{\gamma,i,a} \quad (5r_D r_T^2 N_o N_v) \quad (6297)$$

$$\tau^6_{\gamma,\delta,w} = \sum_{a \in V} {}^2D^3_{a,w} Y^3_{a,\gamma} Y^{3,*}_{a,\delta} \quad (3r_D r_T^2 N_v) \quad (6298)$$

$$\tau^7_{\gamma,\delta,w} = \sum_{i \in O} {}^2D^4_{i,w} Y^4_{i,\gamma} Y^{4,*}_{i,\delta} \quad (3r_D r_T^2 N_o) \quad (6299)$$

$$\tau^8_{\gamma,\delta,w} = \sum_{\epsilon \in A} Z_{\gamma,\epsilon} \tau^6_{\epsilon,\delta,w} \tau^7_{\epsilon,\delta,w} \quad (3r_D r_T^3) \quad (6300)$$

$${}^2R^z_{\gamma,\delta} \leftarrow - \sum_{\epsilon \in A} \sum_{w \in D} \frac{1}{2} \tau^5_{\epsilon,\gamma,w} \tau^8_{\epsilon,\delta,w} \quad (2r_D r_T^3) \quad (6301)$$

Raw expression

$${}^2R^z_{\epsilon,\zeta} \leftarrow - \sum_{i \in O} \sum_{j \in O} \sum_{k \in O} \sum_{a \in V} \sum_{b \in V} \sum_{c \in V} \sum_{d \in V} \frac{1}{2} {}^1T_{a,k} Y^{1,*}_{a,\epsilon} Y^{2,*}_{i,\epsilon} Y^{3,*}_{b,\zeta} Y^{4,*}_{j,\zeta} {}^2D^{a,i,b,j} {}^2T_{c,i,d,j} V_{b,d,k,c} \quad (6302)$$

Factorized expression

$$\tau^0_{\gamma,\delta,w} = \sum_{a \in V} {}^2D^1_{a,w} Y^1_{a,\gamma} Y^{1,*}_{a,\delta} \quad (3r_D r_T^2 N_v) \quad (6303)$$

$$\tau^1_{\gamma,\alpha,w} = \sum_{a \in V} {}^2D^3_{a,w} W^1_{a,\alpha} Y^{3,*}_{a,\gamma} \quad (3r_D r_T r_V N_v) \quad (6304)$$

$$\tau^2_{\gamma,\alpha} = \sum_{a \in V} W^2_{a,\alpha} Y^3_{a,\gamma} \quad (2r_T r_V N_v) \quad (6305)$$

$$\tau^3_{\gamma,\alpha,i} = \sum_{\delta \in A} Z_{\gamma,\delta} Y^4_{i,\delta} \tau^2_{\delta,\alpha} \quad (3r_T^2 r_V N_o) \quad (6306)$$

$$\tau^4_{\gamma,\delta,\alpha,w} = \sum_{i \in O} {}^2D^4_{i,w} Y^{4,*}_{i,\delta} \tau^1_{\delta,\alpha,w} \tau^3_{\gamma,\alpha,i} \quad (4r_D r_T^2 r_V N_o) \quad (6307)$$

$$\tau^5_{\alpha,i} = \sum_{a \in V} {}^1T_{a,i} W^4_{a,\alpha} \quad (2r_V N_o N_v) \quad (6308)$$

$$\tau^6_{\alpha,i,j} = \sum_{\beta \in B} X_{\alpha,\beta} W^3_{j,\beta} \tau^5_{\beta,i} \quad (3r_V^2 N_o^2) \quad (6309)$$

$$\tau^7_{\gamma,\alpha,i} = \sum_{j \in O} Y^2_{j,\gamma} \tau^6_{\alpha,i,j} \quad (2r_T r_V N_o^2) \quad (6310)$$

$$\tau^8_{\gamma,\delta,w,i} = \sum_{\alpha \in B} \tau^7_{\gamma,\alpha,i} \tau^4_{\gamma,\delta,\alpha,w} \quad (2r_D r_T^2 r_V N_o) \quad (6311)$$

$${}^2R^z_{\gamma,\delta} \leftarrow - \sum_{\epsilon \in A} \sum_{w \in D} \sum_{i \in O} \frac{1}{2} {}^2D^2_{i,w} Y^{2,*}_{i,\gamma} \tau^0_{\epsilon,\gamma,w} \tau^8_{\epsilon,\delta,w,i} \quad (4r_D r_T^3 N_o) \quad (6312)$$

Raw expression

$${}^2R^z_{\epsilon,\zeta} \leftarrow - \sum_{i \in O} \sum_{j \in O} \sum_{k \in O} \sum_{a \in V} \sum_{b \in V} \sum_{c \in V} \sum_{d \in V} \frac{1}{2} {}^1T_{a,k} Y^{1,*}_{a,\epsilon} Y^{2,*}_{i,\epsilon} Y^{3,*}_{b,\zeta} Y^{4,*}_{j,\zeta} {}^2D^{a,i,b,j} {}^2T_{c,j,d,i} V_{b,c,k,d} \quad (6313)$$

Factorized expression

$$\tau^0_{\gamma,\delta,w} = \sum_{a \in V} {}^2D^1_{a,w} Y^3_{a,\gamma} Y^{1,*}_{a,\delta} \quad (3r_D r_T^2 N_v) \quad (6314)$$

$$\tau^1_{\gamma,\alpha,w} = \sum_{a \in V} {}^2D^3_{a,w} W^1_{a,\alpha} Y^{3,*}_{a,\gamma} \quad (3r_D r_T r_V N_v) \quad (6315)$$

$$\tau^2_{\gamma,\alpha} = \sum_{a \in V} W^2_{a,\alpha} Y^1_{a,\gamma} \quad (2r_T r_V N_v) \quad (6316)$$

$$\tau^3_{\gamma,\alpha,i} = \sum_{\delta \in A} Y^2_{i,\delta} Z_{\delta,\gamma} \tau^2_{\delta,\alpha} \quad (3r_T^2 r_V N_o) \quad (6317)$$

$$\tau^4_{\gamma,\delta,\alpha,w} = \sum_{i \in O} {}^2D^4_{i,w} Y^{4,*}_{i,\delta} \tau^1_{\delta,\alpha,w} \tau^3_{\gamma,\alpha,i} \quad (4r_D r_T^2 r_V N_o) \quad (6318)$$



$$\tau^5_{\alpha,i} = \sum_{a \in V} {}^1T_{a,i} W^4_{a,\alpha} \quad (2r_V N_o N_v) \quad (6319)$$

$$\tau^7_{\gamma,\delta,w,i} = \sum_{\alpha \in B} \tau^6_{\gamma,\alpha,i} \tau^3_{\gamma,\delta,\alpha,w} \quad (2r_D r_T^2 r_V N_o) \quad (6332)$$

$$\tau^6_{\alpha,i,j} = \sum_{\beta \in B} X_{\alpha,\beta} W^3_{j,\beta} \tau^5_{\beta,i} \quad (3r_V^2 N_o^2) \quad (6320)$$

$$\tau^8_{\gamma,\delta,w} = \sum_{a \in V} {}^2D^3_{a,w} Y^1_{a,\gamma} Y^{3,*}_{a,\delta} \quad (3r_D r_T^2 N_v) \quad (6333)$$

$$\tau^7_{\gamma,\alpha,i} = \sum_{j \in O} Y^4_{j,\gamma} \tau^6_{\alpha,i,j} \quad (2r_T r_V N_o^2) \quad (6321)$$

$${}^2R^z_{\gamma,\delta} \leftarrow - \sum_{\epsilon \in A} \sum_{w \in D} \sum_{i \in O} \frac{1}{2} {}^2D^4_{i,w} Y^{4,*}_{i,\delta} \tau^8_{\epsilon,\delta,w} \tau^7_{\epsilon,\gamma,w,i} \quad (4r_D r_T^3 N_o) \quad (6334)$$

$$\tau^8_{\gamma,\delta,w,i} = \sum_{\alpha \in B} \tau^7_{\gamma,\alpha,i} \tau^4_{\gamma,\delta,\alpha,w} \quad (2r_D r_T^2 r_V N_o) \quad (6322)$$

Raw expression

$${}^2R^z_{\gamma,\delta} \leftarrow - \sum_{\epsilon \in A} \sum_{w \in D} \sum_{i \in O} \frac{1}{2} {}^2D^2_{i,w} Y^{2,*}_{i,\gamma} \tau^0_{\epsilon,\gamma,w} \tau^8_{\epsilon,\delta,w,i} \quad (4r_D r_T^3 N_o) \quad (6323)$$

$${}^2R^z_{\epsilon,\zeta} \leftarrow - \sum_{i \in O} \sum_{j \in O} \sum_{k \in O} \sum_{a \in V} \sum_{b \in V} \sum_{c \in V} \sum_{d \in V} \frac{1}{2} {}^1T_{b,k} Y^{1,*}_{a,\epsilon} Y^{2,*}_{i,\epsilon} Y^{3,*}_{b,\zeta} Y^{4,*}_{j,\zeta} {}^2D^{a,i,b,j} {}^2T_{c,j,d,i} V_{a,d,k,c} \quad (6335)$$

Raw expression

$${}^2R^z_{\epsilon,\zeta} \leftarrow - \sum_{i \in O} \sum_{j \in O} \sum_{k \in O} \sum_{a \in V} \sum_{b \in V} \sum_{c \in V} \sum_{d \in V} \frac{1}{2} {}^1T_{b,k} Y^{1,*}_{a,\epsilon} Y^{2,*}_{i,\epsilon} Y^{3,*}_{b,\zeta} Y^{4,*}_{j,\zeta} {}^2D^{a,i,b,j} {}^2T_{c,i,d,j} V_{a,c,k,d} \quad (6324)$$

Factorized expression

$$\tau^0_{\gamma,\alpha,w} = \sum_{a \in V} {}^2D^1_{a,w} W^1_{a,\alpha} Y^{1,*}_{a,\gamma} \quad (3r_D r_T r_V N_v) \quad (6336)$$

Factorized expression

$$\tau^0_{\gamma,\alpha,w} = \sum_{a \in V} {}^2D^1_{a,w} W^1_{a,\alpha} Y^{1,*}_{a,\gamma} \quad (3r_D r_T r_V N_v) \quad (6325)$$

$$\tau^1_{\gamma,\alpha} = \sum_{a \in V} W^2_{a,\alpha} Y^1_{a,\gamma} \quad (2r_T r_V N_v) \quad (6337)$$

$$\tau^2_{\gamma,\alpha,i} = \sum_{\delta \in A} Y^2_{i,\delta} Z_{\delta,\gamma} \tau^1_{\delta,\alpha} \quad (3r_T^2 r_V N_o) \quad (6338)$$

$$\tau^1_{\gamma,\alpha} = \sum_{a \in V} W^2_{a,\alpha} Y^3_{a,\gamma} \quad (2r_T r_V N_v) \quad (6326)$$

$$\tau^3_{\gamma,\delta,\alpha,w} = \sum_{i \in O} {}^2D^2_{i,w} Y^{2,*}_{i,\delta} \tau^0_{\delta,\alpha,w} \tau^2_{\gamma,\alpha,i} \quad (4r_D r_T^2 r_V N_o) \quad (6339)$$

$$\tau^2_{\gamma,\alpha,i} = \sum_{\delta \in A} Z_{\gamma,\delta} Y^4_{i,\delta} \tau^1_{\delta,\alpha} \quad (3r_T^2 r_V N_o) \quad (6327)$$

$$\tau^4_{\alpha,i} = \sum_{a \in V} {}^1T_{a,i} W^4_{a,\alpha} \quad (2r_V N_o N_v) \quad (6340)$$

$$\tau^3_{\gamma,\delta,\alpha,w} = \sum_{i \in O} {}^2D^2_{i,w} Y^{2,*}_{i,\delta} \tau^0_{\delta,\alpha,w} \tau^2_{\gamma,\alpha,i} \quad (4r_D r_T^2 r_V N_o) \quad (6328)$$

$$\tau^5_{\alpha,i,j} = \sum_{\beta \in B} X_{\alpha,\beta} W^3_{j,\beta} \tau^4_{\beta,i} \quad (3r_V^2 N_o^2) \quad (6341)$$

$$\tau^4_{\alpha,i} = \sum_{a \in V} {}^1T_{a,i} W^4_{a,\alpha} \quad (2r_V N_o N_v) \quad (6329)$$

$$\tau^6_{\gamma,\alpha,i} = \sum_{j \in O} Y^4_{j,\gamma} \tau^5_{\alpha,i,j} \quad (2r_T r_V N_o^2) \quad (6342)$$

$$\tau^5_{\alpha,i,j} = \sum_{\beta \in B} X_{\alpha,\beta} W^3_{j,\beta} \tau^4_{\beta,i} \quad (3r_V^2 N_o^2) \quad (6330)$$

$$\tau^7_{\gamma,\delta,w,i} = \sum_{\alpha \in B} \tau^6_{\gamma,\alpha,i} \tau^3_{\gamma,\delta,\alpha,w} \quad (2r_D r_T^2 r_V N_o) \quad (6343)$$

$$\tau^6_{\gamma,\alpha,i} = \sum_{j \in O} Y^2_{j,\gamma} \tau^5_{\alpha,i,j} \quad (2r_T r_V N_o^2) \quad (6331)$$

$$\tau^8_{\gamma,\delta,w} = \sum_{a \in V} {}^2D^3_{a,w} Y^3_{a,\gamma} Y^{3,*}_{a,\delta} \quad (3r_D r_T^2 N_v) \quad (6344)$$

$${}^2R^z_{\gamma,\delta} \leftarrow - \sum_{\epsilon \in A} \sum_{w \in D} \sum_{i \in O} \frac{1}{2} {}^2D^4_{i,w} Y^{4,*}_{i,\delta} \tau^8_{\epsilon,\delta,w} \tau^7_{\epsilon,\gamma,w,i} \quad (4r_D r_T^3 N_o) \quad (6345)$$

$${}^2R^z_{\epsilon,\zeta} \leftarrow - \sum_{i \in O} \sum_{j \in O} \sum_{k \in O} \sum_{a \in V} \sum_{b \in V} \sum_{c \in V} \sum_{d \in V} \frac{1}{2} {}^1T_{c,i} Y^{1,*}_{a,\epsilon} Y^{2,*}_{i,\epsilon} Y^{3,*}_{b,\zeta} Y^{4,*}_{j,\zeta} {}^2D^{a,i,b,j} {}^2T_{b,j,d,k} V_{a,d,k,c} \quad (6357)$$

Raw expression

$${}^2R^z_{\epsilon,\zeta} \leftarrow - \sum_{i \in O} \sum_{j \in O} \sum_{k \in O} \sum_{a \in V} \sum_{b \in V} \sum_{c \in V} \sum_{d \in V} \frac{1}{2} {}^1T_{c,i} Y^{1,*}_{a,\epsilon} Y^{2,*}_{i,\epsilon} Y^{3,*}_{b,\zeta} Y^{4,*}_{j,\zeta} {}^2D^{a,i,b,j} {}^2T_{a,k,d,j} V_{b,d,k,c} \quad (6346)$$

Factorized expression

$$\tau^0_{\gamma,\delta,w} = \sum_{a \in V} {}^2D^1_{a,w} Y^1_{a,\gamma} Y^{1,*}_{a,\delta} \quad (3r_D r_T^2 N_v) \quad (6347)$$

$$\tau^1_{\gamma,\alpha} = \sum_{i \in O} W^3_{i,\alpha} Y^2_{i,\gamma} \quad (2r_T r_V N_o) \quad (6348)$$

$$\tau^2_{\gamma,\alpha} = \sum_{a \in V} W^4_{a,\alpha} Y^3_{a,\gamma} \quad (2r_T r_V N_v) \quad (6349)$$

$$\tau^3_{\gamma,\alpha,i} = \sum_{\delta \in A} Z_{\gamma,\delta} Y^4_{i,\delta} \tau^2_{\delta,\alpha} \quad (3r_T^2 r_V N_o) \quad (6350)$$

$$\tau^4_{\gamma,\alpha,w} = \sum_{\delta \in A} \sum_{i \in O} {}^2D^2_{i,w} Y^{2,*}_{i,\gamma} \tau^1_{\delta,\alpha} \tau^0_{\delta,\gamma,w} \tau^3_{\delta,\alpha,i} \quad (5r_D r_T^2 r_V N_o) \quad (6351)$$

$$\tau^5_{\gamma,\alpha,w} = \sum_{\beta \in B} X_{\alpha,\beta} \tau^4_{\gamma,\beta,w} \quad (2r_D r_T r_V^2) \quad (6352)$$

$$\tau^6_{\alpha,i} = \sum_{a \in V} {}^1T_{a,i} W^2_{a,\alpha} \quad (2r_V N_o N_v) \quad (6353)$$

$$\tau^7_{\gamma,\alpha,w} = \sum_{i \in O} {}^2D^4_{i,w} Y^{4,*}_{i,\gamma} \tau^6_{\alpha,i} \quad (3r_D r_T r_V N_o) \quad (6354)$$

$$\tau^8_{\gamma,\alpha,w} = \sum_{a \in V} {}^2D^3_{a,w} W^1_{a,\alpha} Y^{3,*}_{a,\gamma} \quad (3r_D r_T r_V N_v) \quad (6355)$$

$${}^2R^z_{\gamma,\delta} \leftarrow - \sum_{\alpha \in B} \sum_{w \in D} \frac{1}{2} \tau^5_{\gamma,\alpha,w} \tau^7_{\delta,\alpha,w} \tau^8_{\delta,\alpha,w} \quad (3r_D r_T^2 r_V) \quad (6356)$$

Raw expression

Factorized expression

$$\tau^0_{\gamma,\delta,w} = \sum_{a \in V} {}^2D^1_{a,w} Y^3_{a,\gamma} Y^{1,*}_{a,\delta} \quad (3r_D r_T^2 N_v) \quad (6358)$$

$$\tau^1_{\gamma,\alpha} = \sum_{a \in V} W^4_{a,\alpha} Y^1_{a,\gamma} \quad (2r_T r_V N_v) \quad (6359)$$

$$\tau^2_{\gamma,\alpha,i} = \sum_{\delta \in A} Y^2_{i,\delta} Z_{\delta,\gamma} \tau^1_{\delta,\alpha} \quad (3r_T^2 r_V N_o) \quad (6360)$$

$$\tau^3_{\gamma,\alpha} = \sum_{i \in O} W^3_{i,\alpha} Y^4_{i,\gamma} \quad (2r_T r_V N_o) \quad (6361)$$

$$\tau^4_{\gamma,\alpha,w} = \sum_{\delta \in A} \sum_{i \in O} {}^2D^2_{i,w} Y^{2,*}_{i,\gamma} \tau^3_{\delta,\alpha} \tau^0_{\delta,\gamma,w} \tau^2_{\delta,\alpha,i} \quad (5r_D r_T^2 r_V N_o) \quad (6362)$$

$$\tau^5_{\gamma,\alpha,w} = \sum_{\beta \in B} X_{\alpha,\beta} \tau^4_{\gamma,\beta,w} \quad (2r_D r_T r_V^2) \quad (6363)$$

$$\tau^6_{\alpha,i} = \sum_{a \in V} {}^1T_{a,i} W^2_{a,\alpha} \quad (2r_V N_o N_v) \quad (6364)$$

$$\tau^7_{\gamma,\alpha,w} = \sum_{i \in O} {}^2D^4_{i,w} Y^{4,*}_{i,\gamma} \tau^6_{\alpha,i} \quad (3r_D r_T r_V N_o) \quad (6365)$$

$$\tau^8_{\gamma,\alpha,w} = \sum_{a \in V} {}^2D^3_{a,w} W^1_{a,\alpha} Y^{3,*}_{a,\gamma} \quad (3r_D r_T r_V N_v) \quad (6366)$$

$${}^2R^z_{\gamma,\delta} \leftarrow - \sum_{\alpha \in B} \sum_{w \in D} \frac{1}{2} \tau^5_{\gamma,\alpha,w} \tau^7_{\delta,\alpha,w} \tau^8_{\delta,\alpha,w} \quad (3r_D r_T^2 r_V) \quad (6367)$$

Raw expression

$${}^2R^z_{\epsilon,\zeta} \leftarrow - \sum_{i \in O} \sum_{j \in O} \sum_{k \in O} \sum_{a \in V} \sum_{b \in V} \sum_{c \in V} \sum_{d \in V} \frac{1}{2} {}^1T_{c,i} Y^{1,*}_{a,\epsilon} Y^{2,*}_{i,\epsilon} Y^{3,*}_{b,\zeta} Y^{4,*}_{j,\zeta} {}^2D^{a,i,b,j} {}^2T_{b,k,d,j} V_{a,c,k,d} \quad (6368)$$

Factorized expression

$$\tau_{\gamma,\delta,w}^0 = \sum_{a \in V} {}^2D_{a,w}^1 Y_{a,\gamma}^1 Y_{a,\delta}^{1,*} \quad (3r_D r_T^2 N_v) \quad (6369)$$

$$\tau_{\gamma,\delta,w}^2 = \sum_{\epsilon \in A} Z_{\gamma,\epsilon} \tau_{\epsilon,\delta,w}^0 \tau_{\epsilon,\delta,w}^1 \quad (3r_D r_T^3) \quad (6382)$$

$$\tau_{\gamma,\delta,w}^1 = \sum_{i \in O} {}^2D_{i,w}^2 Y_{i,\gamma}^2 Y_{i,\delta}^{2,*} \quad (3r_D r_T^2 N_o) \quad (6370)$$

$$\tau_{\alpha,i}^3 = \sum_{a \in V} {}^1T_{a,i} W_{a,\alpha}^4 \quad (2r_V N_o N_v) \quad (6383)$$

$$\tau_{\alpha,i}^2 = \sum_{a \in V} {}^1T_{a,i} W_{a,\alpha}^4 \quad (2r_V N_o N_v) \quad (6371)$$

$$\tau_{\alpha,i,j}^4 = \sum_{\beta \in B} X_{\alpha,\beta} W_{j,\beta}^3 \tau_{\beta,i}^3 \quad (3r_V^2 N_o^2) \quad (6384)$$

$$\tau_{\alpha,i,j}^3 = \sum_{\beta \in B} X_{\alpha,\beta} W_{j,\beta}^3 \tau_{\beta,i}^2 \quad (3r_V^2 N_o^2) \quad (6372)$$

$$\tau_{\gamma,\alpha,i}^5 = \sum_{j \in O} Y_{j,\gamma}^2 \tau_{\alpha,i,j}^4 \quad (2r_T r_V N_o^2) \quad (6385)$$

$$\tau_{\gamma,\alpha,i}^4 = \sum_{j \in O} Y_{j,\gamma}^4 \tau_{\alpha,i,j}^3 \quad (2r_T r_V N_o^2) \quad (6373)$$

$$\tau_{\gamma,\alpha}^6 = \sum_{a \in V} W_{a,\alpha}^2 Y_{a,\gamma}^1 \quad (2r_T r_V N_v) \quad (6386)$$

$$\tau_{\gamma,\alpha}^5 = \sum_{a \in V} W_{a,\alpha}^2 Y_{a,\gamma}^3 \quad (2r_T r_V N_v) \quad (6374)$$

$$\tau_{\gamma,i,a}^7 = \sum_{\alpha \in B} W_{a,\alpha}^1 \tau_{\gamma,\alpha}^6 \tau_{\gamma,\alpha,i}^5 \quad (3r_T r_V N_o N_v) \quad (6387)$$

$$\tau_{\gamma,i,a}^6 = \sum_{\alpha \in B} W_{a,\alpha}^1 \tau_{\gamma,\alpha}^5 \tau_{\gamma,\alpha,i}^4 \quad (3r_T r_V N_o N_v) \quad (6375)$$

$$\tau_{\gamma,\delta,w}^8 = \sum_{i \in O} \sum_{a \in V} {}^2D_{a,w}^3 {}^2D_{i,w}^4 Y_{a,\delta}^{3,*} Y_{i,\delta}^{4,*} \tau_{\gamma,i,a}^7 \quad (5r_D r_T^2 N_o N_v) \quad (6388)$$

$$\tau_{\gamma,\delta,w}^7 = \sum_{i \in O} \sum_{a \in V} {}^2D_{a,w}^3 {}^2D_{i,w}^4 Y_{a,\delta}^{3,*} Y_{i,\delta}^{4,*} \tau_{\gamma,i,a}^6 \quad (5r_D r_T^2 N_o N_v) \quad (6376)$$

$${}^2R_{\gamma,\delta}^z \leftarrow - \sum_{\epsilon \in A} \sum_{w \in D} \frac{1}{2} \tau_{\epsilon,\gamma,w}^2 \tau_{\epsilon,\delta,w}^8 \quad (2r_D r_T^3) \quad (6389)$$

$$\tau_{\gamma,\delta,w}^8 = \sum_{\epsilon \in A} Z_{\gamma,\epsilon} \tau_{\epsilon,\delta,w}^7 \quad (2r_D r_T^3) \quad (6377)$$

Raw expression

$${}^2R_{\gamma,\delta}^z \leftarrow - \sum_{\epsilon \in A} \sum_{w \in D} \frac{1}{2} \tau_{\epsilon,\gamma,w}^0 \tau_{\epsilon,\gamma,w}^1 \tau_{\epsilon,\delta,w}^8 \quad (3r_D r_T^3) \quad (6378)$$

$${}^2R_{\epsilon,\zeta}^z \leftarrow - \sum_{i \in O} \sum_{j \in O} \sum_{k \in O} \sum_{a \in V} \sum_{b \in V} \sum_{c \in V} \sum_{d \in V} \frac{1}{2} {}^1T_{c,i} Y_{a,\epsilon}^{1,*} Y_{i,\epsilon}^{2,*} Y_{b,\zeta}^{3,*} Y_{j,\zeta}^{4,*} {}^2D_{a,i,b,j} {}^2T_{d,j,b,k} V_{a,c,k,d} \quad (6390)$$

Raw expression

$${}^2R_{\epsilon,\zeta}^z \leftarrow - \sum_{i \in O} \sum_{j \in O} \sum_{k \in O} \sum_{a \in V} \sum_{b \in V} \sum_{c \in V} \sum_{d \in V} \frac{1}{2} {}^1T_{c,i} Y_{a,\epsilon}^{1,*} Y_{i,\epsilon}^{2,*} Y_{b,\zeta}^{3,*} Y_{j,\zeta}^{4,*} {}^2D_{a,i,b,j} {}^2T_{d,j,a,k} V_{b,d,k,c} \quad (6379)$$

Factorized expression

$$\tau_{\gamma,\delta,w}^0 = \sum_{i \in O} {}^2D_{i,w}^2 Y_{i,\gamma}^4 Y_{i,\delta}^{2,*} \quad (3r_D r_T^2 N_o) \quad (6391)$$

$$\tau_{\alpha,i}^1 = \sum_{a \in V} {}^1T_{a,i} W_{a,\alpha}^2 \quad (2r_V N_o N_v) \quad (6392)$$

Factorized expression

$$\tau_{\gamma,\delta,w}^0 = \sum_{a \in V} {}^2D_{a,w}^1 Y_{a,\gamma}^3 Y_{a,\delta}^{1,*} \quad (3r_D r_T^2 N_v) \quad (6380)$$

$$\tau_{\alpha,\beta}^2 = \sum_{i \in O} W_{i,\beta}^3 \tau_{\alpha,i}^1 \quad (2r_V^2 N_o) \quad (6393)$$

$$\tau_{\gamma,\delta,w}^1 = \sum_{i \in O} {}^2D_{i,w}^2 Y_{i,\gamma}^4 Y_{i,\delta}^{2,*} \quad (3r_D r_T^2 N_o) \quad (6381)$$

$$\tau_{\alpha,a}^3 = \sum_{\beta \in B} X_{\alpha,\beta} W_{a,\beta}^4 \tau_{\alpha,\beta}^2 \quad (3r_V^2 N_v) \quad (6394)$$

$$\tau^4_{a,b} = \sum_{\alpha \in B} W^1_{a,\alpha} \tau^3_{\alpha,b} \quad (2r_V N_v^2) \quad (6395)$$

$$\tau^5_{\gamma,a} = \sum_{b \in V} Y^1_{b,\gamma} \tau^4_{a,b} \quad (2r_T N_v^2) \quad (6408)$$

$$\tau^5_{\gamma,a} = \sum_{b \in V} Y^3_{b,\gamma} \tau^4_{a,b} \quad (2r_T N_v^2) \quad (6396)$$

$$\tau^6_{\gamma,\delta,w} = \sum_{a \in V} {}^2D^1_{a,w} Y^{1,*}_{a,\delta} \tau^5_{\gamma,a} \quad (3r_D r_T^2 N_v) \quad (6409)$$

$$\tau^6_{\gamma,\delta,w} = \sum_{a \in V} {}^2D^1_{a,w} Y^{1,*}_{a,\delta} \tau^5_{\gamma,a} \quad (3r_D r_T^2 N_v) \quad (6397)$$

$$\tau^7_{\gamma,\delta,w} = \sum_{a \in V} {}^2D^3_{a,w} Y^3_{a,\gamma} Y^{3,*}_{a,\delta} \quad (3r_D r_T^2 N_v) \quad (6410)$$

$$\tau^7_{\gamma,\delta,w} = \sum_{\epsilon \in A} Z_{\gamma,\epsilon} \tau^0_{\epsilon,\delta,w} \tau^6_{\epsilon,\delta,w} \quad (3r_D r_T^3) \quad (6398)$$

$$\tau^8_{\gamma,\delta,w} = \sum_{i \in O} {}^2D^4_{i,w} Y^4_{i,\gamma} Y^{4,*}_{i,\delta} \quad (3r_D r_T^2 N_o) \quad (6411)$$

$$\tau^8_{\gamma,\delta,w} = \sum_{a \in V} {}^2D^3_{a,w} Y^1_{a,\gamma} Y^{3,*}_{a,\delta} \quad (3r_D r_T^2 N_v) \quad (6399)$$

$$\tau^9_{\gamma,\delta,w} = \sum_{\epsilon \in A} Z_{\gamma,\epsilon} \tau^7_{\epsilon,\delta,w} \tau^8_{\epsilon,\delta,w} \quad (3r_D r_T^3) \quad (6412)$$

$$\tau^9_{\gamma,\delta,w} = \sum_{i \in O} {}^2D^4_{i,w} Y^2_{i,\gamma} Y^{4,*}_{i,\delta} \quad (3r_D r_T^2 N_o) \quad (6400)$$

$${}^2R^z_{\gamma,\delta} \leftarrow - \sum_{\epsilon \in A} \sum_{w \in D} \frac{1}{2} \tau^0_{\epsilon,\gamma,w} \tau^6_{\epsilon,\gamma,w} \tau^9_{\epsilon,\delta,w} \quad (3r_D r_T^3) \quad (6413)$$

$${}^2R^z_{\gamma,\delta} \leftarrow - \sum_{\epsilon \in A} \sum_{w \in D} \frac{1}{2} \tau^7_{\epsilon,\gamma,w} \tau^8_{\epsilon,\delta,w} \tau^9_{\epsilon,\delta,w} \quad (3r_D r_T^3) \quad (6401)$$

Raw expression

$${}^2R^z_{\epsilon,\zeta} \leftarrow - \sum_{i \in O} \sum_{j \in O} \sum_{k \in O} \sum_{a \in V} \sum_{b \in V} \sum_{c \in V} \sum_{d \in V} \frac{1}{2} {}^1T_{c,j} Y^{1,*}_{a,\epsilon} Y^{2,*}_{i,\epsilon} Y^{3,*}_{b,\zeta} Y^{4,*}_{j,\zeta} {}^2D^{a,i,b,j} {}^2T_{a,i,d,k} V_{b,d,k,c} \quad (6414)$$

Raw expression

$${}^2R^z_{\epsilon,\zeta} \leftarrow - \sum_{i \in O} \sum_{j \in O} \sum_{k \in O} \sum_{a \in V} \sum_{b \in V} \sum_{c \in V} \sum_{d \in V} \frac{1}{2} {}^1T_{c,i} Y^{1,*}_{a,\epsilon} Y^{2,*}_{i,\epsilon} Y^{3,*}_{b,\zeta} Y^{4,*}_{j,\zeta} {}^2D^{a,i,b,j} {}^2T_{d,k,b,j} V_{a,d,k,c} \quad (6402)$$

Factorized expression

$$\tau^0_{\gamma,\delta,w} = \sum_{i \in O} {}^2D^4_{i,w} Y^4_{i,\gamma} Y^{4,*}_{i,\delta} \quad (3r_D r_T^2 N_o) \quad (6415)$$

Factorized expression

$$\tau^0_{\gamma,\delta,w} = \sum_{i \in O} {}^2D^2_{i,w} Y^2_{i,\gamma} Y^{2,*}_{i,\delta} \quad (3r_D r_T^2 N_o) \quad (6403)$$

$$\tau^1_{\alpha,i} = \sum_{a \in V} {}^1T_{a,i} W^2_{a,\alpha} \quad (2r_V N_o N_v) \quad (6416)$$

$$\tau^1_{\alpha,i} = \sum_{a \in V} {}^1T_{a,i} W^2_{a,\alpha} \quad (2r_V N_o N_v) \quad (6404)$$

$$\tau^2_{\alpha,\beta} = \sum_{i \in O} W^3_{i,\beta} \tau^1_{\alpha,i} \quad (2r_V^2 N_o) \quad (6417)$$

$$\tau^2_{\alpha,\beta} = \sum_{i \in O} W^3_{i,\beta} \tau^1_{\alpha,i} \quad (2r_V^2 N_o) \quad (6405)$$

$$\tau^3_{\alpha,a} = \sum_{\beta \in B} X_{\alpha,\beta} W^4_{a,\beta} \tau^2_{\alpha,\beta} \quad (3r_V^2 N_v) \quad (6418)$$

$$\tau^3_{\alpha,a} = \sum_{\beta \in B} X_{\alpha,\beta} W^4_{a,\beta} \tau^2_{\alpha,\beta} \quad (3r_V^2 N_v) \quad (6406)$$

$$\tau^4_{a,b} = \sum_{\alpha \in B} W^1_{a,\alpha} \tau^3_{\alpha,b} \quad (2r_V N_v^2) \quad (6419)$$

$$\tau^4_{a,b} = \sum_{\alpha \in B} W^1_{a,\alpha} \tau^3_{\alpha,b} \quad (2r_V N_v^2) \quad (6407)$$

$$\tau^5_{\gamma,a} = \sum_{b \in V} Y^3_{b,\gamma} \tau^4_{a,b} \quad (2r_T N_v^2) \quad (6420)$$

$$\tau^6_{\gamma,\delta,w} = \sum_{a \in V} {}^2D^3_{a,w} Y^{3,*}_{a,\delta} \tau^5_{\gamma,a} \quad (3r_D r_T^2 N_v) \quad (6421)$$

$$\tau^7_{\gamma,\delta,w} = \sum_{\epsilon \in A} Z_{\gamma,\epsilon} \tau^0_{\epsilon,\delta,w} \tau^6_{\epsilon,\delta,w} \quad (3r_D r_T^3) \quad (6422)$$

$$\tau^8_{\gamma,\delta,w} = \sum_{a \in V} {}^2D^1_{a,w} Y^1_{a,\gamma} Y^{1,*}_{a,\delta} \quad (3r_D r_T^2 N_v) \quad (6423)$$

$$\tau^9_{\gamma,\delta,w} = \sum_{i \in O} {}^2D^2_{i,w} Y^2_{i,\gamma} Y^{2,*}_{i,\delta} \quad (3r_D r_T^2 N_o) \quad (6424)$$

$${}^2R^z_{\gamma,\delta} \leftarrow - \sum_{\epsilon \in A} \sum_{w \in D} \frac{1}{2} \tau^7_{\epsilon,\delta,w} \tau^8_{\epsilon,\gamma,w} \tau^9_{\epsilon,\gamma,w} \quad (3r_D r_T^3) \quad (6425)$$

Raw expression

$${}^2R^z_{\epsilon,\zeta} \leftarrow - \sum_{i \in O} \sum_{j \in O} \sum_{k \in O} \sum_{a \in V} \sum_{b \in V} \sum_{c \in V} \sum_{d \in V} \frac{1}{2} {}^1T_{c,j} Y^{1,*}_{a,\epsilon} Y^{2,*}_{i,\epsilon} Y^{3,*}_{b,\zeta} Y^{4,*}_{j,\zeta} {}^2D^{a,i,b,j}_{a,k,d,i} {}^2T_{a,k,d,i} V_{b,c,k,d} \quad (6426)$$

Factorized expression

$$\tau^0_{\gamma,\delta,w} = \sum_{i \in O} {}^2D^4_{i,w} Y^2_{i,\gamma} Y^{4,*}_{i,\delta} \quad (3r_D r_T^2 N_o) \quad (6427)$$

$$\tau^1_{\alpha,i} = \sum_{a \in V} {}^1T_{a,i} W^2_{a,\alpha} \quad (2r_V N_o N_v) \quad (6428)$$

$$\tau^2_{\alpha,\beta} = \sum_{i \in O} W^3_{i,\beta} \tau^1_{\alpha,i} \quad (2r_V^2 N_o) \quad (6429)$$

$$\tau^3_{\alpha,a} = \sum_{\beta \in B} X_{\alpha,\beta} W^4_{a,\beta} \tau^2_{\alpha,\beta} \quad (3r_V^2 N_v) \quad (6430)$$

$$\tau^4_{a,b} = \sum_{\alpha \in B} W^1_{a,\alpha} \tau^3_{\alpha,b} \quad (2r_V N_v^2) \quad (6431)$$

$$\tau^5_{\gamma,a} = \sum_{b \in V} Y^1_{b,\gamma} \tau^4_{a,b} \quad (2r_T N_v^2) \quad (6432)$$

$$\tau^6_{\gamma,\delta,w} = \sum_{a \in V} {}^2D^3_{a,w} Y^{3,*}_{a,\delta} \tau^5_{\gamma,a} \quad (3r_D r_T^2 N_v) \quad (6433)$$

$$\tau^7_{\gamma,\delta,w} = \sum_{a \in V} {}^2D^1_{a,w} Y^3_{a,\gamma} Y^{1,*}_{a,\delta} \quad (3r_D r_T^2 N_v) \quad (6434)$$

$$\tau^8_{\gamma,\delta,w} = \sum_{i \in O} {}^2D^2_{i,w} Y^4_{i,\gamma} Y^{2,*}_{i,\delta} \quad (3r_D r_T^2 N_o) \quad (6435)$$

$$\tau^9_{\gamma,\delta,w} = \sum_{\epsilon \in A} Z_{\gamma,\epsilon} \tau^7_{\epsilon,\delta,w} \tau^8_{\epsilon,\delta,w} \quad (3r_D r_T^3) \quad (6436)$$

$${}^2R^z_{\gamma,\delta} \leftarrow - \sum_{\epsilon \in A} \sum_{w \in D} \frac{1}{2} \tau^0_{\epsilon,\delta,w} \tau^6_{\epsilon,\delta,w} \tau^9_{\epsilon,\gamma,w} \quad (3r_D r_T^3) \quad (6437)$$

Raw expression

$${}^2R^z_{\epsilon,\zeta} \leftarrow - \sum_{i \in O} \sum_{j \in O} \sum_{k \in O} \sum_{a \in V} \sum_{b \in V} \sum_{c \in V} \sum_{d \in V} \frac{1}{2} {}^1T_{c,j} Y^{1,*}_{a,\epsilon} Y^{2,*}_{i,\epsilon} Y^{3,*}_{b,\zeta} Y^{4,*}_{j,\zeta} {}^2D^{a,i,b,j}_{a,k,d,i} {}^2T_{b,k,d,i} V_{a,d,k,c} \quad (6438)$$

Factorized expression

$$\tau^0_{\gamma,\delta,w} = \sum_{a \in V} {}^2D^3_{a,w} Y^1_{a,\gamma} Y^{3,*}_{a,\delta} \quad (3r_D r_T^2 N_v) \quad (6439)$$

$$\tau^1_{\gamma,\delta,w} = \sum_{i \in O} {}^2D^4_{i,w} Y^2_{i,\gamma} Y^{4,*}_{i,\delta} \quad (3r_D r_T^2 N_o) \quad (6440)$$

$$\tau^2_{\gamma,w,i} = \sum_{a \in V} {}^2D^1_{a,w} {}^1T_{a,i} Y^{1,*}_{a,\gamma} \quad (3r_D r_T N_o N_v) \quad (6441)$$

$$\tau^3_{\gamma,\alpha,w} = \sum_{i \in O} W^1_{i,\alpha} \tau^2_{\gamma,w,i} \quad (2r_D r_T r_V N_o) \quad (6442)$$

$$\tau^4_{\gamma,\alpha,w} = \sum_{i \in O} {}^2D^2_{i,w} W^2_{i,\alpha} Y^{2,*}_{i,\gamma} \quad (3r_D r_T r_V N_o) \quad (6443)$$

$$\tau^5_{\gamma,\alpha} = \sum_{a \in V} W^4_{a,\alpha} Y^3_{a,\gamma} \quad (2r_T r_V N_v) \quad (6444)$$

$$\tau^6_{\gamma,\alpha} = \sum_{i \in O} W^3_{i,\alpha} Y^4_{i,\gamma} \quad (2r_T r_V N_o) \quad (6445)$$

$$\tau^7_{\gamma,\alpha} = \sum_{\beta \in B} X_{\alpha,\beta} \tau^5_{\gamma,\beta} \tau^6_{\gamma,\beta} \quad (3r_T r_V^2) \quad (6446)$$

$$\tau_{\gamma,\alpha}^8 = \sum_{\delta \in A} Z_{\gamma,\delta} \tau_{\delta,\alpha}^7 \quad (2r_T^2 r_V) \quad (6447)$$

$$\tau_{\gamma,\delta,w}^9 = \sum_{\alpha \in B} \tau_{\gamma,\alpha}^8 \tau_{\delta,\alpha,w}^3 \tau_{\delta,\alpha,w}^4 \quad (3r_D r_T^2 r_V) \quad (6460)$$

$$\tau_{\gamma,\delta,w}^9 = \sum_{\alpha \in B} \tau_{\gamma,\alpha}^8 \tau_{\delta,\alpha,w}^3 \tau_{\delta,\alpha,w}^4 \quad (3r_D r_T^2 r_V) \quad (6448)$$

$${}^2R_{\gamma,\delta}^z \leftarrow - \sum_{\epsilon \in A} \sum_{w \in D} \tau_{\epsilon,\delta,w}^0 \tau_{\epsilon,\delta,w}^1 \tau_{\epsilon,\gamma,w}^9 \quad (3r_D r_T^3) \quad (6461)$$

$${}^2R_{\gamma,\delta}^z \leftarrow - \sum_{\epsilon \in A} \sum_{w \in D} \tau_{\epsilon,\delta,w}^0 \tau_{\epsilon,\delta,w}^1 \tau_{\epsilon,\gamma,w}^9 \quad (3r_D r_T^3) \quad (6449)$$

Raw expression

$${}^2R_{\epsilon,\zeta}^z \leftarrow - \sum_{i \in O} \sum_{j \in O} \sum_{k \in O} \sum_{a \in V} \sum_{b \in V} \sum_{c \in V} \sum_{d \in V} \frac{1}{2} {}^1T_{c,j} Y^{1,*}_{a,\epsilon} Y^{2,*}_{i,\epsilon} Y^{3,*}_{b,\zeta} Y^{4,*}_{j,\zeta} {}^2D^{a,i,b,j} {}^2T_{d,i,b,k} V_{a,d,k,c} \quad (6462)$$

Raw expression

$${}^2R_{\epsilon,\zeta}^z \leftarrow - \sum_{i \in O} \sum_{j \in O} \sum_{k \in O} \sum_{a \in V} \sum_{b \in V} \sum_{c \in V} \sum_{d \in V} \frac{1}{2} {}^1T_{c,j} Y^{1,*}_{a,\epsilon} Y^{2,*}_{i,\epsilon} Y^{3,*}_{b,\zeta} Y^{4,*}_{j,\zeta} {}^2D^{a,i,b,j} {}^2T_{d,i,a,k} V_{b,c,k,d} \quad (6450)$$

Factorized expression

$$\tau_{\gamma,\alpha}^0 = \sum_{a \in V} W_{a,\alpha}^2 Y_{a,\gamma}^3 \quad (2r_T r_V N_v) \quad (6463)$$

Factorized expression

$$\tau_{\gamma,\delta,w}^0 = \sum_{a \in V} {}^2D_{a,w}^3 Y_{a,\gamma}^3 Y_{a,\delta}^{3,*} \quad (3r_D r_T^2 N_v) \quad (6451)$$

$$\tau_{\gamma,\alpha}^1 = \sum_{i \in O} W_{i,\alpha}^1 Y_{i,\gamma}^4 \quad (2r_T r_V N_o) \quad (6464)$$

$$\tau_{\gamma,\delta,w}^1 = \sum_{i \in O} {}^2D_{i,w}^4 Y_{i,\gamma}^4 Y_{i,\delta}^{4,*} \quad (3r_D r_T^2 N_o) \quad (6452)$$

$$\tau_{\gamma,\alpha}^2 = \sum_{\beta \in B} X_{\beta,\alpha} \tau_{\gamma,\beta}^0 \tau_{\gamma,\beta}^1 \quad (3r_T r_V^2) \quad (6465)$$

$$\tau_{\gamma,w,i}^2 = \sum_{a \in V} {}^2D_{a,w}^1 T_{a,i} Y_{a,\gamma}^{1,*} \quad (3r_D r_T N_o N_v) \quad (6453)$$

$$\tau_{\gamma,\alpha}^3 = \sum_{\delta \in A} Z_{\gamma,\delta} \tau_{\delta,\alpha}^2 \quad (2r_T^2 r_V) \quad (6466)$$

$$\tau_{\gamma,\alpha,w}^3 = \sum_{i \in O} W_{i,\alpha}^1 \tau_{\gamma,w,i}^2 \quad (2r_D r_T r_V N_o) \quad (6454)$$

$$\tau_{\gamma,w,i}^4 = \sum_{a \in V} {}^2D_{a,w}^3 T_{a,i} Y_{a,\gamma}^{3,*} \quad (3r_D r_T N_o N_v) \quad (6467)$$

$$\tau_{\gamma,\alpha,w}^4 = \sum_{i \in O} {}^2D_{i,w}^2 W_{i,\alpha}^2 Y_{i,\gamma}^{2,*} \quad (3r_D r_T r_V N_o) \quad (6455)$$

$$\tau_{\gamma,\alpha,w}^5 = \sum_{i \in O} W_{i,\alpha}^3 \tau_{\gamma,w,i}^4 \quad (2r_D r_T r_V N_o) \quad (6468)$$

$$\tau_{\gamma,\alpha}^5 = \sum_{a \in V} W_{a,\alpha}^4 Y_{a,\gamma}^1 \quad (2r_T r_V N_v) \quad (6456)$$

$$\tau_{\gamma,\alpha,w}^6 = \sum_{i \in O} {}^2D_{i,w}^4 W_{i,\alpha}^4 Y_{i,\gamma}^{4,*} \quad (3r_D r_T r_V N_o) \quad (6469)$$

$$\tau_{\gamma,\alpha}^6 = \sum_{i \in O} W_{i,\alpha}^3 Y_{i,\gamma}^2 \quad (2r_T r_V N_o) \quad (6457)$$

$$\tau_{\gamma,\delta,w}^7 = \sum_{\alpha \in B} \tau_{\gamma,\alpha}^3 \tau_{\delta,\alpha,w}^5 \tau_{\delta,\alpha,w}^6 \quad (3r_D r_T^2 r_V) \quad (6470)$$

$$\tau_{\gamma,\alpha}^7 = \sum_{\beta \in B} X_{\alpha,\beta} \tau_{\gamma,\beta}^5 \tau_{\gamma,\beta}^6 \quad (3r_T r_V^2) \quad (6458)$$

$$\tau_{\gamma,\delta,w}^8 = \sum_{a \in V} {}^2D_{a,w}^1 Y_{a,\gamma}^1 Y_{a,\delta}^{1,*} \quad (3r_D r_T^2 N_v) \quad (6471)$$

$$\tau_{\gamma,\alpha}^8 = \sum_{\delta \in A} Z_{\delta,\gamma} \tau_{\delta,\alpha}^7 \quad (2r_T^2 r_V) \quad (6459)$$

$$\tau_{\gamma,\delta,w}^9 = \sum_{i \in O} {}^2D_{i,w}^2 Y_{i,\gamma}^2 Y_{i,\delta}^{2,*} \quad (3r_D r_T^2 N_o) \quad (6472)$$

$${}^2R^z_{\gamma,\delta} \leftarrow - \sum_{\epsilon \in A} \sum_{w \in D} \tau^7_{\epsilon,\delta,w} \tau^8_{\epsilon,\gamma,w} \tau^9_{\epsilon,\gamma,w} \quad (3r_D r_T^3) \quad (6473)$$

Raw expression

$${}^2R^z_{\epsilon,\zeta} \leftarrow - \sum_{i \in O} \sum_{j \in O} \sum_{k \in O} \sum_{a \in V} \sum_{b \in V} \sum_{c \in V} \sum_{d \in V} \frac{1}{2} {}^1T_{c,j} Y^{1,*}_{a,\epsilon} Y^{2,*}_{i,\epsilon} Y^{3,*}_{b,\zeta} Y^{4,*}_{j,\zeta} {}^2D^{a,i,b,j} {}^2T_{d,k,a,i} V_{b,d,k,c} \quad (6474)$$

Factorized expression

$$\tau^0_{\gamma,\alpha} = \sum_{a \in V} W^2_{a,\alpha} Y^1_{a,\gamma} \quad (2r_T r_V N_v) \quad (6475)$$

$$\tau^1_{\gamma,\alpha} = \sum_{i \in O} W^1_{i,\alpha} Y^2_{i,\gamma} \quad (2r_T r_V N_o) \quad (6476)$$

$$\tau^2_{\gamma,\alpha} = \sum_{\beta \in B} X_{\beta,\alpha} \tau^0_{\gamma,\beta} \tau^1_{\gamma,\beta} \quad (3r_T r_V^2) \quad (6477)$$

$$\tau^3_{\gamma,\alpha} = \sum_{\delta \in A} Z_{\delta,\gamma} \tau^2_{\delta,\alpha} \quad (2r_T^2 r_V) \quad (6478)$$

$$\tau^4_{\gamma,w,i} = \sum_{a \in V} {}^2D^3_{a,w} {}^1T_{a,i} Y^{3,*}_{a,\gamma} \quad (3r_D r_T N_o N_v) \quad (6479)$$

$$\tau^5_{\gamma,\alpha,w} = \sum_{i \in O} W^3_{i,\alpha} \tau^4_{\gamma,w,i} \quad (2r_D r_T r_V N_o) \quad (6480)$$

$$\tau^6_{\gamma,\alpha,w} = \sum_{i \in O} {}^2D^4_{i,w} W^4_{i,\alpha} Y^{4,*}_{i,\gamma} \quad (3r_D r_T r_V N_o) \quad (6481)$$

$$\tau^7_{\gamma,\delta,w} = \sum_{\alpha \in B} \tau^3_{\gamma,\alpha} \tau^5_{\delta,\alpha,w} \tau^6_{\delta,\alpha,w} \quad (3r_D r_T^2 r_V) \quad (6482)$$

$$\tau^8_{\gamma,\delta,w} = \sum_{a \in V} {}^2D^1_{a,w} Y^3_{a,\gamma} Y^{1,*}_{a,\delta} \quad (3r_D r_T^2 N_v) \quad (6483)$$

$$\tau^9_{\gamma,\delta,w} = \sum_{i \in O} {}^2D^2_{i,w} Y^4_{i,\gamma} Y^{2,*}_{i,\delta} \quad (3r_D r_T^2 N_o) \quad (6484)$$

$${}^2R^z_{\gamma,\delta} \leftarrow - \sum_{\epsilon \in A} \sum_{w \in D} \tau^7_{\epsilon,\delta,w} \tau^8_{\epsilon,\gamma,w} \tau^9_{\epsilon,\gamma,w} \quad (3r_D r_T^3) \quad (6485)$$

Raw expression

$${}^2R^z_{\epsilon,\zeta} \leftarrow - \sum_{i \in O} \sum_{j \in O} \sum_{k \in O} \sum_{a \in V} \sum_{b \in V} \sum_{c \in V} \sum_{d \in V} \frac{1}{2} {}^1T_{c,k} Y^{1,*}_{a,\epsilon} Y^{2,*}_{i,\epsilon} Y^{3,*}_{b,\zeta} Y^{4,*}_{j,\zeta} {}^2D^{a,i,b,j} {}^2T_{a,i,d,j} V_{b,c,k,d} \quad (6486)$$

Factorized expression

$$\tau^0_{\gamma,\delta,w} = \sum_{a \in V} {}^2D^1_{a,w} Y^1_{a,\gamma} Y^{1,*}_{a,\delta} \quad (3r_D r_T^2 N_v) \quad (6487)$$

$$\tau^1_{\gamma,\delta,w} = \sum_{i \in O} {}^2D^2_{i,w} Y^2_{i,\gamma} Y^{2,*}_{i,\delta} \quad (3r_D r_T^2 N_o) \quad (6488)$$

$$\tau^2_{\gamma,\delta,w} = \sum_{\epsilon \in A} Z_{\epsilon,\gamma} \tau^0_{\epsilon,\delta,w} \tau^1_{\epsilon,\delta,w} \quad (3r_D r_T^3) \quad (6489)$$

$$\tau^3_{\gamma,\delta,w} = \sum_{a \in V} {}^2D^3_{a,w} Y^3_{a,\gamma} Y^{3,*}_{a,\delta} \quad (3r_D r_T^2 N_v) \quad (6490)$$

$$\tau^4_{\alpha,i} = \sum_{a \in V} {}^1T_{a,i} W^2_{a,\alpha} \quad (2r_V N_o N_v) \quad (6491)$$

$$\tau^5_{\alpha} = \sum_{i \in O} W^1_{i,\alpha} \tau^4_{\alpha,i} \quad (2r_V N_o) \quad (6492)$$

$$\tau^6_{\alpha} = \sum_{\beta \in B} \tau^5_{\beta} X_{\beta,\alpha} \quad (2r_V^2) \quad (6493)$$

$$\tau^7_{i,j} = \sum_{\alpha \in B} \tau^6_{\alpha} W^3_{i,\alpha} W^4_{j,\alpha} \quad (3r_V N_o^2) \quad (6494)$$

$$\tau^8_{\gamma,i} = \sum_{j \in O} Y^4_{j,\gamma} \tau^7_{j,i} \quad (2r_T N_o^2) \quad (6495)$$

$$\tau^9_{\gamma,\delta,w} = \sum_{i \in O} {}^2D^4_{i,w} Y^{4,*}_{i,\delta} \tau^8_{\gamma,i} \quad (3r_D r_T^2 N_o) \quad (6496)$$

$${}^2R^z_{\gamma,\delta} \leftarrow - \sum_{\epsilon \in A} \sum_{w \in D} \tau^2_{\epsilon,\gamma,w} \tau^3_{\epsilon,\delta,w} \tau^9_{\epsilon,\delta,w} \quad (3r_D r_T^3) \quad (6497)$$

Raw expression

$${}^2R^z_{\epsilon,\zeta} \leftarrow - \sum_{i \in O} \sum_{j \in O} \sum_{k \in O} \sum_{a \in V} \sum_{b \in V} \sum_{c \in V} \sum_{d \in V} \frac{1}{2} {}^1T_{c,k} Y^{1,*}_{a,\epsilon} Y^{2,*}_{i,\epsilon} Y^{3,*}_{b,\zeta} Y^{4,*}_{j,\zeta} {}^2D^{a,i,b,j} {}^2T_{b,j,d,i} V_{a,c,k,d} \quad (6498)$$

Factorized expression

$$\tau_{\gamma,\delta,w}^0 = \sum_{a \in V} {}^2D_{a,w}^1 Y_{a,\gamma}^3 Y_{a,\delta}^{1,*} \quad (3r_D r_T^2 N_v) \quad (6499)$$

$$\tau_{\gamma,\delta,w}^1 = \sum_{i \in O} {}^2D_{i,w}^2 Y_{i,\gamma}^4 Y_{i,\delta}^{2,*} \quad (3r_D r_T^2 N_o) \quad (6500)$$

$$\tau_{\gamma,\delta,w}^2 = \sum_{a \in V} {}^2D_{a,w}^3 Y_{a,\gamma}^1 Y_{a,\delta}^{3,*} \quad (3r_D r_T^2 N_v) \quad (6501)$$

$$\tau_{\alpha,i}^3 = \sum_{a \in V} {}^1T_{a,i} W_{a,\alpha}^2 \quad (2r_V N_o N_v) \quad (6502)$$

$$\tau_{\alpha}^4 = \sum_{i \in O} W_{i,\alpha}^1 \tau_{\alpha,i}^3 \quad (2r_V N_o) \quad (6503)$$

$$\tau_{\alpha}^5 = \sum_{\beta \in B} \tau_{\beta,\alpha}^4 X_{\beta,\alpha} \quad (2r_V^2) \quad (6504)$$

$$\tau_{i,j}^6 = \sum_{\alpha \in B} \tau_{\alpha}^5 W_{i,\alpha}^3 W_{j,\alpha}^4 \quad (3r_V N_o^2) \quad (6505)$$

$$\tau_{\gamma,i}^7 = \sum_{j \in O} Y_{j,\gamma}^2 \tau_{j,i}^6 \quad (2r_T N_o^2) \quad (6506)$$

$$\tau_{\gamma,\delta,w}^8 = \sum_{i \in O} {}^2D_{i,w}^4 Y_{i,\delta}^{4,*} \tau_{\gamma,i}^7 \quad (3r_D r_T^2 N_o) \quad (6507)$$

$$\tau_{\gamma,\delta,w}^9 = \sum_{\epsilon \in A} Z_{\epsilon,\gamma} \tau_{\epsilon,\delta,w}^2 \tau_{\epsilon,\delta,w}^8 \quad (3r_D r_T^3) \quad (6508)$$

$${}^2R_{\gamma,\delta}^z \leftarrow - \sum_{\epsilon \in A} \sum_{w \in D} \tau_{\epsilon,\gamma,w}^0 \tau_{\epsilon,\gamma,w}^1 \tau_{\epsilon,\delta,w}^9 \quad (3r_D r_T^3) \quad (6509)$$

Raw expression

$${}^2R_{\epsilon,\zeta}^z \leftarrow - \sum_{i \in O} \sum_{j \in O} \sum_{k \in O} \sum_{a \in V} \sum_{b \in V} \sum_{c \in V} \sum_{d \in V} \frac{1}{2} {}^1T_{c,k} Y_{a,\epsilon}^{1,*} Y_{i,\epsilon}^{2,*} Y_{b,\zeta}^{3,*} Y_{j,\zeta}^{4,*} {}^2D_{a,i,b,j} {}^2T_{d,i,b,j} V_{a,c,k,d} \quad (6510)$$

Factorized expression

$$\tau_{\gamma,\delta,w}^0 = \sum_{a \in V} {}^2D_{a,w}^3 Y_{a,\gamma}^3 Y_{a,\delta}^{3,*} \quad (3r_D r_T^2 N_v) \quad (6511)$$

$$\tau_{\gamma,\delta,w}^1 = \sum_{i \in O} {}^2D_{i,w}^4 Y_{i,\gamma}^4 Y_{i,\delta}^{4,*} \quad (3r_D r_T^2 N_o) \quad (6512)$$

$$\tau_{\gamma,\delta,w}^2 = \sum_{a \in V} {}^2D_{a,w}^1 Y_{a,\gamma}^1 Y_{a,\delta}^{1,*} \quad (3r_D r_T^2 N_v) \quad (6513)$$

$$\tau_{\alpha,i}^3 = \sum_{a \in V} {}^1T_{a,i} W_{a,\alpha}^4 \quad (2r_V N_o N_v) \quad (6514)$$

$$\tau_{\alpha}^4 = \sum_{i \in O} W_{i,\alpha}^3 \tau_{\alpha,i}^3 \quad (2r_V N_o) \quad (6515)$$

$$\tau_{\alpha}^5 = \sum_{\beta \in B} \tau_{\beta,\alpha}^4 X_{\alpha,\beta} \quad (2r_V^2) \quad (6516)$$

$$\tau_{i,j}^6 = \sum_{\alpha \in B} \tau_{\alpha}^5 W_{i,\alpha}^1 W_{j,\alpha}^2 \quad (3r_V N_o^2) \quad (6517)$$

$$\tau_{\gamma,i}^7 = \sum_{j \in O} Y_{j,\gamma}^2 \tau_{j,i}^6 \quad (2r_T N_o^2) \quad (6518)$$

$$\tau_{\gamma,\delta,w}^8 = \sum_{i \in O} {}^2D_{i,w}^2 Y_{i,\delta}^{2,*} \tau_{\gamma,i}^7 \quad (3r_D r_T^2 N_o) \quad (6519)$$

$$\tau_{\gamma,\delta,w}^9 = \sum_{\epsilon \in A} Z_{\epsilon,\gamma} \tau_{\epsilon,\delta,w}^2 \tau_{\epsilon,\delta,w}^8 \quad (3r_D r_T^3) \quad (6520)$$

$${}^2R_{\gamma,\delta}^z \leftarrow - \sum_{\epsilon \in A} \sum_{w \in D} \tau_{\epsilon,\delta,w}^0 \tau_{\epsilon,\delta,w}^1 \tau_{\epsilon,\gamma,w}^9 \quad (3r_D r_T^3) \quad (6521)$$

Raw expression

$${}^2R_{\epsilon,\zeta}^z \leftarrow - \sum_{i \in O} \sum_{j \in O} \sum_{k \in O} \sum_{a \in V} \sum_{b \in V} \sum_{c \in V} \sum_{d \in V} \frac{1}{2} {}^1T_{c,k} Y_{a,\epsilon}^{1,*} Y_{i,\epsilon}^{2,*} Y_{b,\zeta}^{3,*} Y_{j,\zeta}^{4,*} {}^2D_{a,i,b,j} {}^2T_{d,j,a,i} V_{b,c,k,d} \quad (6522)$$

Factorized expression

$$\tau_{\gamma,\delta,w}^0 = \sum_{a \in V} {}^2D_{a,w}^3 Y_{a,\gamma}^1 Y_{a,\delta}^{3,*} \quad (3r_D r_T^2 N_v) \quad (6523)$$

$$\tau_{\gamma,\delta,w}^1 = \sum_{i \in O} {}^2D_{i,w}^4 Y_{i,\gamma}^2 Y_{i,\delta}^{4,*} \quad (3r_D r_T^2 N_o) \quad (6524)$$



$$\tau^2_{\gamma,\delta,w} = \sum_{\epsilon \in A} Z_{\epsilon,\gamma} \tau^0_{\epsilon,\delta,w} \tau^1_{\epsilon,\delta,w} \quad (3r_D r_T^3) \quad (6525)$$

$$\tau^3_{\gamma,\delta,w} = \sum_{a \in V} {}^2D^3_{a,w} Y^1_{a,\gamma} Y^{3,*}_{a,\delta} \quad (3r_D r_T^2 N_v) \quad (6538)$$

$$\tau^3_{\gamma,\delta,w} = \sum_{a \in V} {}^2D^1_{a,w} Y^3_{a,\gamma} Y^{1,*}_{a,\delta} \quad (3r_D r_T^2 N_v) \quad (6526)$$

$$\tau^4_{\alpha,i,j} = \sum_{\beta \in B} X_{\alpha,\beta} W^3_{i,\beta} W^4_{j,\beta} \quad (3r_V^2 N_o^2) \quad (6539)$$

$$\tau^4_{\alpha,i} = \sum_{a \in V} {}^1T_{a,i} W^4_{a,\alpha} \quad (2r_V N_o N_v) \quad (6527)$$

$$\tau^5_{\gamma,\alpha,i} = \sum_{j \in O} Y^2_{j,\gamma} \tau^4_{\alpha,j,i} \quad (2r_T r_V N_o^2) \quad (6540)$$

$$\tau^5_{\alpha} = \sum_{i \in O} W^3_{i,\alpha} \tau^4_{\alpha,i} \quad (2r_V N_o) \quad (6528)$$

$$\tau^6_{\gamma,\delta,\alpha,w} = \sum_{i \in O} {}^2D^4_{i,w} Y^{4,*}_{i,\delta} \tau^3_{\gamma,\delta,w} \tau^5_{\gamma,\alpha,i} \quad (4r_D r_T^2 r_V N_o) \quad (6541)$$

$$\tau^6_{\alpha} = \sum_{\beta \in B} \tau^5_{\beta} X_{\alpha,\beta} \quad (2r_V^2) \quad (6529)$$

$$\tau^7_{\gamma,\alpha,w,i} = \sum_{\delta \in A} \tau^2_{\delta,\alpha,i} \tau^6_{\delta,\gamma,\alpha,w} \quad (2r_D r_T^2 r_V N_o) \quad (6542)$$

$$\tau^7_{i,j} = \sum_{\alpha \in B} \tau^6_{\alpha} W^1_{i,\alpha} W^2_{j,\alpha} \quad (3r_V N_o^2) \quad (6530)$$

$$\tau^8_{\gamma,w,i,j} = \sum_{\alpha \in B} W^1_{i,\alpha} \tau^7_{\gamma,\alpha,w,j} \quad (2r_D r_T r_V N_o^2) \quad (6543)$$

$$\tau^8_{\gamma,i} = \sum_{j \in O} Y^4_{j,\gamma} \tau^7_{j,i} \quad (2r_T N_o^2) \quad (6531)$$

$$\tau^9_{\gamma,\delta,w} = \sum_{i \in O} {}^2D^2_{i,w} Y^{2,*}_{i,\delta} \tau^8_{\gamma,i} \quad (3r_D r_T^2 N_o) \quad (6532)$$

$${}^2R^z_{\gamma,\delta} \leftarrow \sum_{w \in D} \sum_{i \in O} \sum_{j \in O} \frac{1}{2} {}^2D^2_{i,w} Y^{2,*}_{i,\gamma} \tau^0_{\gamma,w,j} \tau^8_{\delta,w,j,i} \quad (4r_D r_T^2 N_o^2) \quad (6544)$$

$${}^2R^z_{\gamma,\delta} \leftarrow - \sum_{\epsilon \in A} \sum_{w \in D} \tau^2_{\epsilon,\delta,w} \tau^3_{\epsilon,\gamma,w} \tau^9_{\epsilon,\gamma,w} \quad (3r_D r_T^3) \quad (6533)$$

Raw expression

$${}^2R^z_{\epsilon,\zeta} \leftarrow \sum_{i \in O} \sum_{j \in O} \sum_{k \in O} \sum_{l \in O} \sum_{a \in V} \sum_{b \in V} \sum_{c \in V} \frac{1}{2} {}^1T_{a,k} Y^{1,*}_{a,\epsilon} Y^{2,*}_{i,\epsilon} Y^{3,*}_{b,\zeta} Y^{4,*}_{j,\zeta} {}^2D^{a,i,b,j} {}^2T_{b,l,c,i} V_{k,c,l,j} \quad (6545)$$

Raw expression

$${}^2R^z_{\epsilon,\zeta} \leftarrow \sum_{i \in O} \sum_{j \in O} \sum_{k \in O} \sum_{l \in O} \sum_{a \in V} \sum_{b \in V} \sum_{c \in V} \frac{1}{2} {}^1T_{a,k} Y^{1,*}_{a,\epsilon} Y^{2,*}_{i,\epsilon} Y^{3,*}_{b,\zeta} Y^{4,*}_{j,\zeta} {}^2D^{a,i,b,j} {}^2T_{b,j,c,l} V_{l,i,k,c} \quad (6534)$$

Factorized expression

$$\tau^0_{\gamma,w,i} = \sum_{a \in V} {}^2D^1_{a,w} {}^1T_{a,i} Y^{1,*}_{a,\gamma} \quad (3r_D r_T N_o N_v) \quad (6546)$$

Factorized expression

$$\tau^0_{\gamma,w,i} = \sum_{a \in V} {}^2D^1_{a,w} {}^1T_{a,i} Y^{1,*}_{a,\gamma} \quad (3r_D r_T N_o N_v) \quad (6535)$$

$$\tau^1_{\gamma,\delta,w} = \sum_{a \in V} {}^2D^3_{a,w} Y^3_{a,\gamma} Y^{3,*}_{a,\delta} \quad (3r_D r_T^2 N_v) \quad (6547)$$

$$\tau^1_{\gamma,\alpha} = \sum_{a \in V} W^2_{a,\alpha} Y^3_{a,\gamma} \quad (2r_T r_V N_v) \quad (6536)$$

$$\tau^2_{\alpha,i,j} = \sum_{\beta \in B} X_{\alpha,\beta} W^3_{i,\beta} W^4_{j,\beta} \quad (3r_V^2 N_o^2) \quad (6548)$$

$$\tau^2_{\gamma,\alpha,i} = \sum_{\delta \in A} Z_{\gamma,\delta} Y^4_{i,\delta} \tau^1_{\delta,\alpha} \quad (3r_T^2 r_V N_o) \quad (6537)$$

$$\tau^3_{\gamma,\alpha,i} = \sum_{j \in O} Y^4_{j,\gamma} \tau^2_{\alpha,j,i} \quad (2r_T r_V N_o^2) \quad (6549)$$

$$\tau^4_{\gamma,\delta,\alpha,w} = \sum_{i \in O} {}^2D^4_{i,w} Y^{4,*}_{i,\delta} \tau^1_{\gamma,\delta,w} \tau^3_{\gamma,\alpha,i} \quad (4r_D r_T^2 r_V N_o) \quad (6550)$$

$$\tau^6_{\gamma,w,i} = \sum_{a \in V} {}^2D^1_{a,w} {}^1T_{a,i} Y^{1,*}_{a,\gamma} \quad (3r_D r_T N_o N_v) \quad (6563)$$

$$\tau^5_{\gamma,\alpha} = \sum_{a \in V} W^2_{a,\alpha} Y^1_{a,\gamma} \quad (2r_T r_V N_v) \quad (6551)$$

$$\tau^7_{\gamma,\alpha,w} = \sum_{i \in O} W^1_{i,\alpha} \tau^6_{\gamma,w,i} \quad (2r_D r_T r_V N_o) \quad (6564)$$

$$\tau^6_{\gamma,\alpha,i} = \sum_{\delta \in A} Y^2_{i,\delta} Z_{\delta,\gamma} \tau^5_{\delta,\alpha} \quad (3r_T^2 r_V N_o) \quad (6552)$$

$$\tau^8_{\gamma,\alpha,w} = \sum_{i \in O} {}^2D^2_{i,w} W^2_{i,\alpha} Y^{2,*}_{i,\gamma} \quad (3r_D r_T r_V N_o) \quad (6565)$$

$$\tau^7_{\gamma,\alpha,w,i} = \sum_{\delta \in A} \tau^6_{\delta,\alpha,i} \tau^4_{\delta,\gamma,\alpha,w} \quad (2r_D r_T^2 r_V N_o) \quad (6553)$$

$${}^2R^z_{\gamma,\delta} \leftarrow \sum_{\alpha \in B} \sum_{w \in D} \frac{1}{2} \tau^5_{\delta,\alpha,w} \tau^7_{\gamma,\alpha,w} \tau^8_{\gamma,\alpha,w} \quad (3r_D r_T^2 r_V) \quad (6566)$$

$$\tau^8_{\gamma,w,i,j} = \sum_{\alpha \in B} W^1_{i,\alpha} \tau^7_{\gamma,\alpha,w,j} \quad (2r_D r_T r_V N_o^2) \quad (6554)$$

Raw expression

$${}^2R^z_{\gamma,\delta} \leftarrow \sum_{w \in D} \sum_{i \in O} \sum_{j \in O} \frac{1}{2} {}^2D^2_{i,w} Y^{2,*}_{i,\gamma} \tau^0_{\gamma,w,j} \tau^8_{\delta,w,j,i} \quad (4r_D r_T^2 r_V N_o^2) \quad (6555)$$

$${}^2R^z_{\gamma,\delta} \leftarrow \sum_{i \in O} \sum_{j \in O} \sum_{k \in O} \sum_{l \in O} \sum_{a \in V} \sum_{b \in V} \sum_{c \in V} \frac{1}{2} {}^1T_{a,k} Y^{1,*}_{a,\epsilon} Y^{2,*}_{i,\epsilon} Y^{3,*}_{b,\zeta} Y^{4,*}_{j,\zeta} {}^2D^{a,i,b,j} {}^2T_{c,i,b,l} V_{k,c,l,j} \quad (6567)$$

Raw expression

$${}^2R^z_{\epsilon,\zeta} \leftarrow \sum_{i \in O} \sum_{j \in O} \sum_{k \in O} \sum_{l \in O} \sum_{a \in V} \sum_{b \in V} \sum_{c \in V} \frac{1}{2} {}^1T_{a,k} Y^{1,*}_{a,\epsilon} Y^{2,*}_{i,\epsilon} Y^{3,*}_{b,\zeta} Y^{4,*}_{j,\zeta} {}^2D^{a,i,b,j} {}^2T_{b,l,c,j} V_{k,i,l,c} \quad (6556)$$

Factorized expression

$$\tau^0_{\gamma,\delta,w} = \sum_{a \in V} {}^2D^3_{a,w} Y^3_{a,\gamma} Y^{3,*}_{a,\delta} \quad (3r_D r_T^2 N_v) \quad (6568)$$

Factorized expression

$$\tau^1_{\gamma,\alpha} = \sum_{a \in V} W^4_{a,\alpha} Y^1_{a,\gamma} \quad (2r_T r_V N_v) \quad (6569)$$

$$\tau^0_{\gamma,\delta,w} = \sum_{a \in V} {}^2D^3_{a,w} Y^1_{a,\gamma} Y^{3,*}_{a,\delta} \quad (3r_D r_T^2 N_v) \quad (6557)$$

$$\tau^2_{\gamma,\alpha,i} = \sum_{\delta \in A} Y^2_{i,\delta} Z_{\delta,\gamma} \tau^1_{\delta,\alpha} \quad (3r_T^2 r_V N_o) \quad (6570)$$

$$\tau^1_{\gamma,\alpha} = \sum_{i \in O} W^3_{i,\alpha} Y^2_{i,\gamma} \quad (2r_T r_V N_o) \quad (6558)$$

$$\tau^3_{\gamma,\alpha} = \sum_{i \in O} W^3_{i,\alpha} Y^4_{i,\gamma} \quad (2r_T r_V N_o) \quad (6571)$$

$$\tau^2_{\gamma,\alpha} = \sum_{a \in V} W^4_{a,\alpha} Y^3_{a,\gamma} \quad (2r_T r_V N_v) \quad (6559)$$

$$\tau^4_{\gamma,\alpha,w} = \sum_{\delta \in A} \sum_{i \in O} {}^2D^4_{i,w} Y^{4,*}_{i,\gamma} \tau^3_{\delta,\alpha} \tau^0_{\delta,\gamma,w} \tau^2_{\delta,\alpha,i} \quad (5r_D r_T^2 r_V N_o) \quad (6572)$$

$$\tau^3_{\gamma,\alpha,i} = \sum_{\delta \in A} Z_{\gamma,\delta} Y^4_{i,\delta} \tau^2_{\delta,\alpha} \quad (3r_T^2 r_V N_o) \quad (6560)$$

$$\tau^4_{\gamma,\alpha,w} = \sum_{\delta \in A} \sum_{i \in O} {}^2D^4_{i,w} Y^{4,*}_{i,\gamma} \tau^1_{\delta,\alpha} \tau^0_{\delta,\gamma,w} \tau^3_{\delta,\alpha,i} \quad (5r_D r_T^2 r_V N_o) \quad (6561)$$

$$\tau^5_{\gamma,\alpha,w} = \sum_{\beta \in B} X_{\alpha,\beta} \tau^4_{\gamma,\beta,w} \quad (2r_D r_T r_V^2) \quad (6573)$$

$$\tau^5_{\gamma,\alpha,w} = \sum_{\beta \in B} X_{\alpha,\beta} \tau^4_{\gamma,\beta,w} \quad (2r_D r_T r_V^2) \quad (6562)$$

$$\tau^6_{\gamma,w,i} = \sum_{a \in V} {}^2D^1_{a,w} {}^1T_{a,i} Y^{1,*}_{a,\gamma} \quad (3r_D r_T N_o N_v) \quad (6574)$$

$$\tau^7_{\gamma,\alpha,w} = \sum_{i \in O} W^1_{i,\alpha} \tau^6_{\gamma,w,i} \quad (2r_D r_T r_V N_o) \quad (6575)$$

$$\tau^8_{\gamma,\alpha,w} = \sum_{i \in O} {}^2D^2_{i,w} W^2_{i,\alpha} Y^{2,*}_{i,\gamma} \quad (3r_D r_T r_V N_o) \quad (6576)$$

$${}^2R^z_{\gamma,\delta} \leftarrow \sum_{\alpha \in B} \sum_{w \in D} \frac{1}{2} \tau^5_{\delta,\alpha,w} \tau^7_{\gamma,\alpha,w} \tau^8_{\gamma,\alpha,w} \quad (3r_D r_T^2 r_V) \quad (6577)$$

Raw expression

$${}^2R^z_{\epsilon,\zeta} \leftarrow \sum_{i \in O} \sum_{j \in O} \sum_{k \in O} \sum_{l \in O} \sum_{a \in V} \sum_{b \in V} \sum_{c \in V} \frac{1}{2} {}^1T_{a,k} Y^{1,*}_{a,\epsilon} Y^{2,*}_{i,\epsilon} Y^{3,*}_{b,\zeta} Y^{4,*}_{j,\zeta} {}^2D^{a,i,b,j} {}^2T_{c,j,b,l} V_{k,i,l,c} \quad (6578)$$

Factorized expression

$$\tau^0_{\gamma,\delta,w} = \sum_{a \in V} {}^2D^3_{a,w} Y^1_{a,\gamma} Y^{3,*}_{a,\delta} \quad (3r_D r_T^2 N_v) \quad (6579)$$

$$\tau^1_{\gamma,\delta,w} = \sum_{i \in O} {}^2D^4_{i,w} Y^2_{i,\gamma} Y^{4,*}_{i,\delta} \quad (3r_D r_T^2 N_o) \quad (6580)$$

$$\tau^2_{\gamma,w,i} = \sum_{a \in V} {}^2D^1_{a,w} {}^1T_{a,i} Y^{1,*}_{a,\gamma} \quad (3r_D r_T N_o N_v) \quad (6581)$$

$$\tau^3_{\alpha,i,j} = \sum_{\beta \in B} W^1_{i,\beta} W^2_{j,\beta} X_{\beta,\alpha} \quad (3r_V^2 N_o^2) \quad (6582)$$

$$\tau^4_{\gamma,\alpha,i} = \sum_{j \in O} Y^4_{j,\gamma} \tau^3_{\alpha,j,i} \quad (2r_T r_V N_o^2) \quad (6583)$$

$$\tau^5_{\gamma,\alpha} = \sum_{a \in V} W^4_{a,\alpha} Y^3_{a,\gamma} \quad (2r_T r_V N_v) \quad (6584)$$

$$\tau^6_{\gamma,i,j} = \sum_{\alpha \in B} W^3_{j,\alpha} \tau^5_{\gamma,\alpha} \tau^4_{\gamma,\alpha,i} \quad (3r_T r_V N_o^2) \quad (6585)$$

$$\tau^7_{\gamma,i,j} = \sum_{\delta \in A} Z_{\gamma,\delta} \tau^6_{\delta,i,j} \quad (2r_T^2 N_o^2) \quad (6586)$$

$$\tau^8_{\gamma,\delta,w} = \sum_{i \in O} \sum_{j \in O} {}^2D^2_{i,w} Y^{2,*}_{i,\delta} \tau^2_{\delta,w,j} \tau^7_{\gamma,i,j} \quad (4r_D r_T^2 N_o^2) \quad (6587)$$

$${}^2R^z_{\gamma,\delta} \leftarrow \sum_{\epsilon \in A} \sum_{w \in D} \frac{1}{2} \tau^0_{\epsilon,\delta,w} \tau^1_{\epsilon,\delta,w} \tau^8_{\epsilon,\gamma,w} \quad (3r_D r_T^3) \quad (6588)$$

Raw expression

$${}^2R^z_{\epsilon,\zeta} \leftarrow \sum_{i \in O} \sum_{j \in O} \sum_{k \in O} \sum_{l \in O} \sum_{a \in V} \sum_{b \in V} \sum_{c \in V} \frac{1}{2} {}^1T_{a,k} Y^{1,*}_{a,\epsilon} Y^{2,*}_{i,\epsilon} Y^{3,*}_{b,\zeta} Y^{4,*}_{j,\zeta} {}^2D^{a,i,b,j} {}^2T_{c,l,b,j} V_{l,i,k,c} \quad (6589)$$

Factorized expression

$$\tau^0_{\gamma,\delta,w} = \sum_{a \in V} {}^2D^3_{a,w} Y^3_{a,\gamma} Y^{3,*}_{a,\delta} \quad (3r_D r_T^2 N_v) \quad (6590)$$

$$\tau^1_{\gamma,\delta,w} = \sum_{i \in O} {}^2D^4_{i,w} Y^4_{i,\gamma} Y^{4,*}_{i,\delta} \quad (3r_D r_T^2 N_o) \quad (6591)$$

$$\tau^2_{\gamma,w,i} = \sum_{a \in V} {}^2D^1_{a,w} {}^1T_{a,i} Y^{1,*}_{a,\gamma} \quad (3r_D r_T N_o N_v) \quad (6592)$$

$$\tau^3_{\alpha,i,j} = \sum_{\beta \in B} W^1_{i,\beta} W^2_{j,\beta} X_{\beta,\alpha} \quad (3r_V^2 N_o^2) \quad (6593)$$

$$\tau^4_{\gamma,\alpha,i} = \sum_{j \in O} Y^2_{j,\gamma} \tau^3_{\alpha,j,i} \quad (2r_T r_V N_o^2) \quad (6594)$$

$$\tau^5_{\gamma,\alpha} = \sum_{a \in V} W^4_{a,\alpha} Y^1_{a,\gamma} \quad (2r_T r_V N_v) \quad (6595)$$

$$\tau^6_{\gamma,i,j} = \sum_{\alpha \in B} W^3_{j,\alpha} \tau^5_{\gamma,\alpha} \tau^4_{\gamma,\alpha,i} \quad (3r_T r_V N_o^2) \quad (6596)$$

$$\tau^7_{\gamma,i,j} = \sum_{\delta \in A} Z_{\delta,\gamma} \tau^6_{\delta,i,j} \quad (2r_T^2 N_o^2) \quad (6597)$$

$$\tau^8_{\gamma,\delta,w} = \sum_{i \in O} \sum_{j \in O} {}^2D^2_{i,w} Y^{2,*}_{i,\delta} \tau^2_{\delta,w,j} \tau^7_{\gamma,i,j} \quad (4r_D r_T^2 N_o^2) \quad (6598)$$

$${}^2R^z_{\gamma,\delta} \leftarrow \sum_{\epsilon \in A} \sum_{w \in D} \frac{1}{2} \tau^0_{\epsilon,\delta,w} \tau^1_{\epsilon,\delta,w} \tau^8_{\epsilon,\gamma,w} \quad (3r_D r_T^3) \quad (6599)$$

Raw expression

$${}^2R^z_{\epsilon,\zeta} \leftarrow \sum_{i \in O} \sum_{j \in O} \sum_{k \in O} \sum_{l \in O} \sum_{a \in V} \sum_{b \in V} \sum_{c \in V} \frac{1}{2} {}^1T_{b,k} {}^{Y^{1,*}}_{a,\epsilon} {}^{Y^{2,*}}_{i,\epsilon} {}^{Y^{3,*}}_{b,\zeta} {}^{Y^{4,*}}_{j,\zeta} {}^2D^{a,i,b,j} {}^2T_{a,i,c,l} V_{k,c,l,j} \quad (6600)$$

Factorized expression

$$\tau^0_{\gamma,w,i} = \sum_{a \in V} {}^2D^3_{a,w} {}^1T_{a,i} {}^{Y^{3,*}}_{a,\gamma} \quad (3r_D r_T N_o N_v) \quad (6601)$$

$$\tau^1_{\gamma,\alpha} = \sum_{a \in V} W^2_{a,\alpha} Y^3_{a,\gamma} \quad (2r_T r_V N_v) \quad (6602)$$

$$\tau^2_{\alpha,i,j} = \sum_{\beta \in B} X_{\alpha,\beta} W^3_{i,\beta} W^4_{j,\beta} \quad (3r_V^2 N_o^2) \quad (6603)$$

$$\tau^3_{\gamma,\alpha,i} = \sum_{j \in O} Y^4_{j,\gamma} \tau^2_{\alpha,j,i} \quad (2r_T r_V N_o^2) \quad (6604)$$

$$\tau^4_{\gamma,i,j} = \sum_{\alpha \in B} W^1_{i,\alpha} \tau^1_{\gamma,\alpha} \tau^3_{\gamma,\alpha,j} \quad (3r_T r_V N_o^2) \quad (6605)$$

$$\tau^5_{\gamma,i,j} = \sum_{\delta \in A} Z_{\gamma,\delta} \tau^4_{\delta,i,j} \quad (2r_T^2 N_o^2) \quad (6606)$$

$$\tau^6_{\gamma,\delta,w} = \sum_{i \in O} \sum_{j \in O} {}^2D^4_{i,w} Y^{4,*}_{i,\delta} \tau^0_{\delta,w,j} \tau^5_{\gamma,j,i} \quad (4r_D r_T^2 N_o^2) \quad (6607)$$

$$\tau^7_{\gamma,\delta,w} = \sum_{a \in V} {}^2D^1_{a,w} Y^1_{a,\gamma} Y^{1,*}_{a,\delta} \quad (3r_D r_T^2 N_v) \quad (6608)$$

$$\tau^8_{\gamma,\delta,w} = \sum_{i \in O} {}^2D^2_{i,w} Y^2_{i,\gamma} Y^{2,*}_{i,\delta} \quad (3r_D r_T^2 N_o) \quad (6609)$$

$${}^2R^z_{\gamma,\delta} \leftarrow \sum_{\epsilon \in A} \sum_{w \in D} \frac{1}{2} \tau^6_{\epsilon,\delta,w} \tau^7_{\epsilon,\gamma,w} \tau^8_{\epsilon,\gamma,w} \quad (3r_D r_T^3) \quad (6610)$$

Raw expression

$${}^2R^z_{\epsilon,\zeta} \leftarrow \sum_{i \in O} \sum_{j \in O} \sum_{k \in O} \sum_{l \in O} \sum_{a \in V} \sum_{b \in V} \sum_{c \in V} \frac{1}{2} {}^1T_{b,k} {}^{Y^{1,*}}_{a,\epsilon} {}^{Y^{2,*}}_{i,\epsilon} {}^{Y^{3,*}}_{b,\zeta} {}^{Y^{4,*}}_{j,\zeta} {}^2D^{a,i,b,j} {}^2T_{a,l,c,i} V_{l,c,k,j} \quad (6611)$$

Factorized expression

$$\tau^0_{\gamma,w,i} = \sum_{a \in V} {}^2D^3_{a,w} {}^1T_{a,i} {}^{Y^{3,*}}_{a,\gamma} \quad (3r_D r_T N_o N_v) \quad (6612)$$

$$\tau^1_{\gamma,\alpha} = \sum_{a \in V} W^2_{a,\alpha} Y^1_{a,\gamma} \quad (2r_T r_V N_v) \quad (6613)$$

$$\tau^2_{\alpha,i,j} = \sum_{\beta \in B} X_{\alpha,\beta} W^3_{i,\beta} W^4_{j,\beta} \quad (3r_V^2 N_o^2) \quad (6614)$$

$$\tau^3_{\gamma,\alpha,i} = \sum_{j \in O} Y^2_{j,\gamma} \tau^2_{\alpha,j,i} \quad (2r_T r_V N_o^2) \quad (6615)$$

$$\tau^4_{\gamma,i,j} = \sum_{\alpha \in B} W^1_{i,\alpha} \tau^1_{\gamma,\alpha} \tau^3_{\gamma,\alpha,j} \quad (3r_T r_V N_o^2) \quad (6616)$$

$$\tau^5_{\gamma,i,j} = \sum_{\delta \in A} Z_{\delta,\gamma} \tau^4_{\delta,i,j} \quad (2r_T^2 N_o^2) \quad (6617)$$

$$\tau^6_{\gamma,\delta,w} = \sum_{i \in O} \sum_{j \in O} {}^2D^4_{i,w} Y^{4,*}_{i,\delta} \tau^0_{\delta,w,j} \tau^5_{\gamma,j,i} \quad (4r_D r_T^2 N_o^2) \quad (6618)$$

$$\tau^7_{\gamma,\delta,w} = \sum_{a \in V} {}^2D^1_{a,w} Y^3_{a,\gamma} Y^{1,*}_{a,\delta} \quad (3r_D r_T^2 N_v) \quad (6619)$$

$$\tau^8_{\gamma,\delta,w} = \sum_{i \in O} {}^2D^2_{i,w} Y^4_{i,\gamma} Y^{2,*}_{i,\delta} \quad (3r_D r_T^2 N_o) \quad (6620)$$

$${}^2R^z_{\gamma,\delta} \leftarrow \sum_{\epsilon \in A} \sum_{w \in D} \frac{1}{2} \tau^6_{\epsilon,\delta,w} \tau^7_{\epsilon,\gamma,w} \tau^8_{\epsilon,\gamma,w} \quad (3r_D r_T^3) \quad (6621)$$

Raw expression

$${}^2R^z_{\epsilon,\zeta} \leftarrow \sum_{i \in O} \sum_{j \in O} \sum_{k \in O} \sum_{l \in O} \sum_{a \in V} \sum_{b \in V} \sum_{c \in V} \frac{1}{2} {}^1T_{b,k} {}^{Y^{1,*}}_{a,\epsilon} {}^{Y^{2,*}}_{i,\epsilon} {}^{Y^{3,*}}_{b,\zeta} {}^{Y^{4,*}}_{j,\zeta} {}^2D^{a,i,b,j} {}^2T_{a,l,c,j} V_{l,i,k,c} \quad (6622)$$

Factorized expression

$$\tau^0_{\gamma,w,i} = \sum_{a \in V} {}^2D^3_{a,w} {}^1T_{a,i} {}^{Y^{3,*}}_{a,\gamma} \quad (3r_D r_T N_o N_v) \quad (6623)$$

$$\tau^1_{\gamma,\alpha,w} = \sum_{i \in O} W^3_{i,\alpha} \tau^0_{\gamma,w,i} \quad (2r_D r_T r_V N_o) \quad (6624)$$

$$\tau^2_{\gamma,\alpha,w} = \sum_{i \in O} {}^2D^4_{i,w} W^4_{i,\alpha} Y^{4,*}_{i,\gamma} \quad (3r_D r_T r_V N_o) \quad (6636)$$

$$\tau^2_{\gamma,\alpha,w} = \sum_{i \in O} {}^2D^4_{i,w} W^4_{i,\alpha} Y^{4,*}_{i,\gamma} \quad (3r_D r_T r_V N_o) \quad (6625)$$

$$\tau^3_{\gamma,\alpha,w} = \sum_{\beta \in B} X_{\alpha,\beta} \tau^1_{\gamma,\beta,w} \tau^2_{\gamma,\beta,w} \quad (3r_D r_T r_V^2) \quad (6637)$$

$$\tau^3_{\gamma,\alpha,w} = \sum_{\beta \in B} X_{\alpha,\beta} \tau^1_{\gamma,\beta,w} \tau^2_{\gamma,\beta,w} \quad (3r_D r_T r_V^2) \quad (6626)$$

$$\tau^4_{\gamma,\delta,w} = \sum_{a \in V} {}^2D^1_{a,w} Y^3_{a,\gamma} Y^{1,*}_{a,\delta} \quad (3r_D r_T^2 N_v) \quad (6638)$$

$$\tau^4_{\gamma,\delta,w} = \sum_{a \in V} {}^2D^1_{a,w} Y^1_{a,\gamma} Y^{1,*}_{a,\delta} \quad (3r_D r_T^2 N_v) \quad (6627)$$

$$\tau^5_{\gamma,\alpha} = \sum_{a \in V} W^2_{a,\alpha} Y^1_{a,\gamma} \quad (2r_T r_V N_o) \quad (6639)$$

$$\tau^5_{\gamma,\alpha} = \sum_{i \in O} W^1_{i,\alpha} Y^2_{i,\gamma} \quad (2r_T r_V N_o) \quad (6628)$$

$$\tau^6_{\gamma,\alpha,i} = \sum_{\delta \in A} Y^2_{i,\delta} Z_{\delta,\gamma} \tau^5_{\delta,\alpha} \quad (3r_T^2 r_V N_o) \quad (6640)$$

$$\tau^6_{\gamma,\alpha} = \sum_{a \in V} W^2_{a,\alpha} Y^3_{a,\gamma} \quad (2r_T r_V N_o) \quad (6629)$$

$$\tau^7_{\gamma,\alpha} = \sum_{i \in O} W^1_{i,\alpha} Y^4_{i,\gamma} \quad (2r_T r_V N_o) \quad (6641)$$

$$\tau^7_{\gamma,\alpha,i} = \sum_{\delta \in A} Z_{\gamma,\delta} Y^4_{i,\delta} \tau^6_{\delta,\alpha} \quad (3r_T^2 r_V N_o) \quad (6630)$$

$$\tau^8_{\gamma,\alpha,w} = \sum_{\delta \in A} \sum_{i \in O} {}^2D^2_{i,w} Y^{2,*}_{i,\gamma} \tau^7_{\delta,\alpha} \tau^4_{\delta,\gamma,w} \tau^6_{\delta,\alpha,i} \quad (5r_D r_T^2 r_V N_o) \quad (6642)$$

$$\tau^8_{\gamma,\alpha,w} = \sum_{\delta \in A} \sum_{i \in O} {}^2D^2_{i,w} Y^{2,*}_{i,\gamma} \tau^5_{\delta,\alpha} \tau^4_{\delta,\gamma,w} \tau^7_{\delta,\alpha,i} \quad (5r_D r_T^2 r_V N_o) \quad (6631)$$

Raw expression

$${}^2R^z_{\gamma,\delta} \leftarrow \sum_{\alpha \in B} \sum_{w \in D} \frac{1}{2} \tau^3_{\delta,\alpha,w} \tau^8_{\gamma,\alpha,w} \quad (2r_D r_T^2 r_V) \quad (6632)$$

$${}^2R^z_{\epsilon,\zeta} \leftarrow \sum_{i \in O} \sum_{j \in O} \sum_{k \in O} \sum_{l \in O} \sum_{a \in V} \sum_{b \in V} \sum_{c \in V} \frac{1}{2} {}^1T_{b,k} Y^{1,*}_{a,\epsilon} Y^{2,*}_{i,\epsilon} Y^{3,*}_{b,\zeta} Y^{4,*}_{j,\zeta} {}^2D^{a,i,b,j} {}^2T_{c,j,a,l} V_{l,i,k,c} \quad (6644)$$

Raw expression

$${}^2R^z_{\epsilon,\zeta} \leftarrow \sum_{i \in O} \sum_{j \in O} \sum_{k \in O} \sum_{l \in O} \sum_{a \in V} \sum_{b \in V} \sum_{c \in V} \frac{1}{2} {}^1T_{b,k} Y^{1,*}_{a,\epsilon} Y^{2,*}_{i,\epsilon} Y^{3,*}_{b,\zeta} Y^{4,*}_{j,\zeta} {}^2D^{a,i,b,j} {}^2T_{c,i,a,l} V_{l,c,k,j} \quad (6633)$$

Factorized expression

Factorized expression

$$\tau^0_{\gamma,w,i} = \sum_{a \in V} {}^2D^3_{a,w} {}^1T_{a,i} Y^{3,*}_{a,\gamma} \quad (3r_D r_T N_o N_v) \quad (6634)$$

$$\tau^0_{\gamma,\delta,w} = \sum_{a \in V} {}^2D^1_{a,w} Y^1_{a,\gamma} Y^{1,*}_{a,\delta} \quad (3r_D r_T^2 N_v) \quad (6645)$$

$$\tau^1_{\alpha,i,j} = \sum_{\beta \in B} W^1_{i,\beta} W^2_{j,\beta} X_{\beta,\alpha} \quad (3r_V^2 N_o^2) \quad (6646)$$

$$\tau^2_{\gamma,\alpha,i} = \sum_{j \in O} Y^2_{j,\gamma} \tau^1_{\alpha,j,i} \quad (2r_T r_V N_o^2) \quad (6647)$$

$$\tau^1_{\gamma,\alpha,w} = \sum_{i \in O} W^3_{i,\alpha} \tau^0_{\gamma,w,i} \quad (2r_D r_T r_V N_o) \quad (6635)$$

$$\tau^3_{\gamma,\delta,\alpha,w} = \sum_{i \in O} {}^2D^2_{i,w} Y^{2,*}_{i,\delta} \tau^0_{\gamma,\delta,w} \tau^2_{\gamma,\alpha,i} \quad (4r_D r_T^2 r_V N_o) \quad (6648)$$

$$\tau^4_{\gamma,\alpha} = \sum_{a \in V} W^4_{a,\alpha} Y^3_{a,\gamma} \quad (2r_T r_V N_v) \quad (6649)$$

$$\tau^6_{\gamma,\alpha,w,i} = \sum_{\delta \in A} \tau^5_{\delta,\alpha,i} \tau^3_{\delta,\gamma,\alpha,w} \quad (2r_D r_T^2 r_V N_o) \quad (6662)$$

$$\tau^5_{\gamma,\alpha,i} = \sum_{\delta \in A} Z_{\gamma,\delta} Y^4_{i,\delta} \tau^4_{\delta,\alpha} \quad (3r_T^2 r_V N_o) \quad (6650)$$

$$\tau^7_{\gamma,w,i,j} = \sum_{\alpha \in B} W^3_{i,\alpha} \tau^6_{\gamma,\alpha,w,j} \quad (2r_D r_T r_V N_o^2) \quad (6663)$$

$$\tau^6_{\gamma,\alpha,w,i} = \sum_{\delta \in A} \tau^5_{\delta,\alpha,i} \tau^3_{\delta,\gamma,\alpha,w} \quad (2r_D r_T^2 r_V N_o) \quad (6651)$$

$$\tau^8_{\gamma,w,i} = \sum_{a \in V} {}^2D^3_{a,w} {}^1T_{a,i} Y^{3,*}_{a,\gamma} \quad (3r_D r_T N_o N_v) \quad (6664)$$

$$\tau^7_{\gamma,w,i,j} = \sum_{\alpha \in B} W^3_{i,\alpha} \tau^6_{\gamma,\alpha,w,j} \quad (2r_D r_T r_V N_o^2) \quad (6652)$$

$$\tau^8_{\gamma,w,i} = \sum_{a \in V} {}^2D^3_{a,w} {}^1T_{a,i} Y^{3,*}_{a,\gamma} \quad (3r_D r_T N_o N_v) \quad (6653)$$

$${}^2R^z_{\gamma,\delta} \leftarrow \sum_{w \in D} \sum_{i \in O} \sum_{j \in O} \frac{1}{2} {}^2D^4_{i,w} Y^{4,*}_{i,\delta} \tau^8_{\delta,w,j} \tau^7_{\gamma,w,j,i} \quad (4r_D r_T^2 N_o^2) \quad (6665)$$

Raw expression

$${}^2R^z_{\gamma,\delta} \leftarrow \sum_{w \in D} \sum_{i \in O} \sum_{j \in O} \frac{1}{2} {}^2D^4_{i,w} Y^{4,*}_{i,\delta} \tau^8_{\delta,w,j} \tau^7_{\gamma,w,j,i} \quad (4r_D r_T^2 N_o^2) \quad (6654)$$

$${}^2R^z_{N_o^2} \leftarrow \sum_{i \in O} \sum_{j \in O} \sum_{k \in O} \sum_{l \in O} \sum_{a \in V} \sum_{b \in V} \sum_{c \in V} \frac{1}{2} {}^1T_{c,i} Y^{1,*}_{a,\epsilon} Y^{2,*}_{i,\epsilon} Y^{3,*}_{b,\zeta} Y^{4,*}_{j,\zeta} {}^2D^{a,i,b,j} {}^2T_{a,k,b,l} V_{k,c,l,j} \quad (6666)$$

Raw expression

$${}^2R^z_{\epsilon,\zeta} \leftarrow \sum_{i \in O} \sum_{j \in O} \sum_{k \in O} \sum_{l \in O} \sum_{a \in V} \sum_{b \in V} \sum_{c \in V} \frac{1}{2} {}^1T_{b,k} Y^{1,*}_{a,\epsilon} Y^{2,*}_{i,\epsilon} Y^{3,*}_{b,\zeta} Y^{4,*}_{j,\zeta} {}^2D^{a,i,b,j} {}^2T_{c,l,a,i} V_{k,c,l,j} \quad (6655)$$

Factorized expression

$$\tau^0_{\gamma,\delta,w} = \sum_{a \in V} {}^2D^1_{a,w} Y^1_{a,\gamma} Y^{1,*}_{a,\delta} \quad (3r_D r_T^2 N_v) \quad (6667)$$

Factorized expression

$$\tau^0_{\gamma,\delta,w} = \sum_{a \in V} {}^2D^1_{a,w} Y^3_{a,\gamma} Y^{1,*}_{a,\delta} \quad (3r_D r_T^2 N_v) \quad (6656)$$

$$\tau^1_{\gamma,\alpha,w} = \sum_{i \in O} {}^2D^4_{i,w} W^4_{i,\alpha} Y^{4,*}_{i,\gamma} \quad (3r_D r_T r_V N_o) \quad (6668)$$

$$\tau^1_{\alpha,i,j} = \sum_{\beta \in B} W^1_{i,\beta} W^2_{j,\beta} X_{\beta,\alpha} \quad (3r_V^2 N_o^2) \quad (6657)$$

$$\tau^2_{\gamma,\delta,w} = \sum_{a \in V} {}^2D^3_{a,w} Y^3_{a,\gamma} Y^{3,*}_{a,\delta} \quad (3r_D r_T^2 N_v) \quad (6669)$$

$$\tau^2_{\gamma,\alpha,i} = \sum_{j \in O} Y^4_{j,\gamma} \tau^1_{\alpha,j,i} \quad (2r_T r_V N_o^2) \quad (6658)$$

$$\tau^3_{\gamma,\delta,w,i} = \sum_{\epsilon \in A} Z_{\gamma,\epsilon} Y^4_{i,\epsilon} \tau^2_{\epsilon,\delta,w} \quad (3r_D r_T^3 N_o) \quad (6670)$$

$$\tau^3_{\gamma,\delta,\alpha,w} = \sum_{i \in O} {}^2D^2_{i,w} Y^{2,*}_{i,\delta} \tau^0_{\gamma,\delta,w} \tau^2_{\gamma,\alpha,i} \quad (4r_D r_T^2 r_V N_o) \quad (6659)$$

$$\tau^4_{\gamma,\delta,\alpha,w} = \sum_{i \in O} W^3_{i,\alpha} \tau^1_{\delta,\alpha,w} \tau^3_{\gamma,\delta,w,i} \quad (3r_D r_T^2 r_V N_o) \quad (6671)$$

$$\tau^4_{\gamma,\alpha} = \sum_{a \in V} W^4_{a,\alpha} Y^1_{a,\gamma} \quad (2r_T r_V N_v) \quad (6660)$$

$$\tau^5_{\alpha,i} = \sum_{a \in V} {}^1T_{a,i} W^2_{a,\alpha} \quad (2r_V N_o N_v) \quad (6672)$$

$$\tau^5_{\gamma,\alpha,i} = \sum_{\delta \in A} Y^2_{i,\delta} Z_{\delta,\gamma} \tau^4_{\delta,\alpha} \quad (3r_T^2 r_V N_o) \quad (6661)$$

$$\tau^6_{\alpha,i,j} = \sum_{\beta \in B} W^1_{j,\beta} X_{\beta,\alpha} \tau^5_{\beta,i} \quad (3r_V^2 N_o^2) \quad (6673)$$

$$\tau^7_{\gamma,\alpha,i} = \sum_{j \in O} Y^2_{j,\gamma} \tau^6_{\alpha,i,j} \quad (2r_T r_V N_o^2) \quad (6674)$$

$${}^2R^z_{\gamma,\delta} \leftarrow \sum_{\epsilon \in A} \sum_{w \in D} \sum_{i \in O} \frac{1}{2} {}^2D^2_{i,w} Y^{2,*}_{i,\gamma} \tau^0_{\epsilon,\gamma,w} \tau^8_{\epsilon,\delta,w,i} \quad (4r_D r_T^3 N_o) \quad (6687)$$

$$\tau^8_{\gamma,\delta,w,i} = \sum_{\alpha \in B} \tau^7_{\gamma,\alpha,i} \tau^4_{\gamma,\delta,\alpha,w} \quad (2r_D r_T^2 r_V N_o) \quad (6675)$$

Raw expression

$${}^2R^z_{\gamma,\delta} \leftarrow \sum_{\epsilon \in A} \sum_{w \in D} \sum_{i \in O} \frac{1}{2} {}^2D^2_{i,w} Y^{2,*}_{i,\gamma} \tau^0_{\epsilon,\gamma,w} \tau^8_{\epsilon,\delta,w,i} \quad (4r_D r_T^3 N_o) \quad (6676)$$

Raw expression

$${}^2R^z_{\epsilon,\zeta} \leftarrow \sum_{i \in O} \sum_{j \in O} \sum_{k \in O} \sum_{l \in O} \sum_{a \in V} \sum_{b \in V} \sum_{c \in V} \frac{1}{2} {}^1T_{c,i} Y^{1,*}_{a,\epsilon} Y^{2,*}_{i,\epsilon} Y^{3,*}_{b,\zeta} Y^{4,*}_{j,\zeta} {}^2D^{a,i,b,j} {}^2T_{b,k,a,l} V_{l,c,k,j} \quad (6677)$$

Factorized expression

$$\tau^0_{\gamma,\delta,w} = \sum_{a \in V} {}^2D^1_{a,w} Y^3_{a,\gamma} Y^{1,*}_{a,\delta} \quad (3r_D r_T^2 N_v) \quad (6678)$$

$$\tau^1_{\gamma,\alpha,w} = \sum_{i \in O} {}^2D^4_{i,w} W^4_{i,\alpha} Y^{4,*}_{i,\gamma} \quad (3r_D r_T r_V N_o) \quad (6679)$$

$$\tau^2_{\gamma,\delta,w} = \sum_{a \in V} {}^2D^3_{a,w} Y^1_{a,\gamma} Y^{3,*}_{a,\delta} \quad (3r_D r_T^2 N_v) \quad (6680)$$

$$\tau^3_{\gamma,\delta,w,i} = \sum_{\epsilon \in A} Y^2_{i,\epsilon} Z_{\epsilon,\gamma} \tau^2_{\epsilon,\delta,w} \quad (3r_D r_T^3 N_o) \quad (6681)$$

$$\tau^4_{\gamma,\delta,\alpha,w} = \sum_{i \in O} W^3_{i,\alpha} \tau^1_{\delta,\alpha,w} \tau^3_{\gamma,\delta,w,i} \quad (3r_D r_T^2 r_V N_o) \quad (6682)$$

$$\tau^5_{\alpha,i} = \sum_{a \in V} {}^1T_{a,i} W^2_{a,\alpha} \quad (2r_V N_o N_v) \quad (6683)$$

$$\tau^6_{\alpha,i,j} = \sum_{\beta \in B} W^1_{j,\beta} X_{\beta,\alpha} \tau^5_{\beta,i} \quad (3r_V^2 N_o^2) \quad (6684)$$

$$\tau^7_{\gamma,\alpha,i} = \sum_{j \in O} Y^4_{j,\gamma} \tau^6_{\alpha,i,j} \quad (2r_T r_V N_o^2) \quad (6685)$$

$$\tau^8_{\gamma,\delta,w,i} = \sum_{\alpha \in B} \tau^7_{\gamma,\alpha,i} \tau^4_{\gamma,\delta,\alpha,w} \quad (2r_D r_T^2 r_V N_o) \quad (6686)$$

Factorized expression

$$\tau^0_{\gamma,\delta,w} = \sum_{a \in V} {}^2D^1_{a,w} Y^1_{a,\gamma} Y^{1,*}_{a,\delta} \quad (3r_D r_T^2 N_v) \quad (6689)$$

$$\tau^1_{\alpha,i} = \sum_{a \in V} {}^1T_{a,i} W^4_{a,\alpha} \quad (2r_V N_o N_v) \quad (6690)$$

$$\tau^2_{\gamma,\alpha,w} = \sum_{i \in O} {}^2D^4_{i,w} Y^{4,*}_{i,\gamma} \tau^1_{\alpha,i} \quad (3r_D r_T r_V N_o) \quad (6691)$$

$$\tau^3_{\gamma,\delta,w} = \sum_{a \in V} {}^2D^3_{a,w} Y^3_{a,\gamma} Y^{3,*}_{a,\delta} \quad (3r_D r_T^2 N_v) \quad (6692)$$

$$\tau^4_{\gamma,\delta,w,i} = \sum_{\epsilon \in A} Z_{\gamma,\epsilon} Y^4_{i,\epsilon} \tau^3_{\epsilon,\delta,w} \quad (3r_D r_T^3 N_o) \quad (6693)$$

$$\tau^5_{\gamma,\delta,\alpha,w} = \sum_{i \in O} W^3_{i,\alpha} \tau^2_{\delta,\alpha,w} \tau^4_{\gamma,\delta,w,i} \quad (3r_D r_T^2 r_V N_o) \quad (6694)$$

$$\tau^6_{\alpha,i,j} = \sum_{\beta \in B} W^1_{i,\beta} W^2_{j,\beta} X_{\beta,\alpha} \quad (3r_V^2 N_o^2) \quad (6695)$$

$$\tau^7_{\gamma,\alpha,i} = \sum_{j \in O} Y^2_{j,\gamma} \tau^6_{\alpha,j,i} \quad (2r_T r_V N_o^2) \quad (6696)$$

$$\tau^8_{\gamma,\delta,w,i} = \sum_{\alpha \in B} \tau^7_{\gamma,\alpha,i} \tau^5_{\gamma,\delta,\alpha,w} \quad (2r_D r_T^2 r_V N_o) \quad (6697)$$

$${}^2R^z_{\gamma,\delta} \leftarrow \sum_{\epsilon \in A} \sum_{w \in D} \sum_{i \in O} \frac{1}{2} {}^2D^2_{i,w} Y^{2,*}_{i,\gamma} \tau^0_{\epsilon,\gamma,w} \tau^8_{\epsilon,\delta,w,i} \quad (4r_D r_T^3 N_o) \quad (6698)$$

Raw expression

$${}^2R^z_{\epsilon,\zeta} \leftarrow \sum_{i \in O} \sum_{j \in O} \sum_{k \in O} \sum_{l \in O} \sum_{a \in V} \sum_{b \in V} \sum_{c \in V} \frac{1}{2} {}^1T_{c,j} Y^{1,*}_{a,\epsilon} Y^{2,*}_{i,\epsilon} Y^{3,*}_{b,\zeta} Y^{4,*}_{j,\zeta} {}^2D^{a,i,b,j} {}^2T_{b,k,a,l} V_{l,i,k,c} \quad (6699)$$

Factorized expression

$$\tau^0_{\gamma,\delta,w} = \sum_{a \in V} {}^2D^1_{a,w} Y^3_{a,\gamma} Y^{1,*}_{a,\delta} \quad (3r_D r_T^2 N_v) \quad (6700)$$

$$\tau^1_{\alpha,i} = \sum_{a \in V} {}^1T_{a,i} W^4_{a,\alpha} \quad (2r_V N_o N_v) \quad (6701)$$

$$\tau^2_{\gamma,\alpha,w} = \sum_{i \in O} {}^2D^4_{i,w} Y^{4,*}_{i,\gamma} \tau^1_{\alpha,i} \quad (3r_D r_T r_V N_o) \quad (6702)$$

$$\tau^3_{\gamma,\delta,w} = \sum_{a \in V} {}^2D^3_{a,w} Y^1_{a,\gamma} Y^{3,*}_{a,\delta} \quad (3r_D r_T^2 N_v) \quad (6703)$$

$$\tau^4_{\gamma,\delta,w,i} = \sum_{\epsilon \in A} Y^2_{i,\epsilon} Z_{\epsilon,\gamma} \tau^3_{\epsilon,\delta,w} \quad (3r_D r_T^3 N_o) \quad (6704)$$

$$\tau^5_{\gamma,\delta,\alpha,w} = \sum_{i \in O} W^3_{i,\alpha} \tau^2_{\delta,\alpha,w} \tau^4_{\gamma,\delta,w,i} \quad (3r_D r_T^2 r_V N_o) \quad (6705)$$

$$\tau^6_{\alpha,i,j} = \sum_{\beta \in B} W^1_{i,\beta} W^2_{j,\beta} X_{\beta,\alpha} \quad (3r_V^2 N_o^2) \quad (6706)$$

$$\tau^7_{\gamma,\alpha,i} = \sum_{j \in O} Y^4_{j,\gamma} \tau^6_{\alpha,j,i} \quad (2r_T r_V N_o^2) \quad (6707)$$

$$\tau^8_{\gamma,\delta,w,i} = \sum_{\alpha \in B} \tau^7_{\gamma,\alpha,i} \tau^5_{\gamma,\delta,\alpha,w} \quad (2r_D r_T^2 r_V N_o) \quad (6708)$$

$${}^2R^z_{\gamma,\delta} \leftarrow \sum_{\epsilon \in A} \sum_{w \in D} \sum_{i \in O} \frac{1}{2} {}^2D^2_{i,w} Y^{2,*}_{i,\gamma} \tau^0_{\epsilon,\gamma,w} \tau^8_{\epsilon,\delta,w,i} \quad (4r_D r_T^3 N_o^2) \quad (6709)$$

Raw expression

$${}^2R^z_{\epsilon,\zeta} \leftarrow \sum_{i \in O} \sum_{j \in O} \sum_{k \in O} \sum_{l \in O} \sum_{a \in V} \sum_{b \in V} \sum_{c \in V} \frac{1}{2} {}^1T_{c,k} Y^{1,*}_{a,\epsilon} Y^{2,*}_{i,\epsilon} Y^{3,*}_{b,\zeta} Y^{4,*}_{j,\zeta} {}^2D^{a,i,b,j} {}^2T_{a,i,b,l} V_{l,c,k,j} \quad (6710)$$

Factorized expression

$$\tau^0_{\gamma,\delta,w} = \sum_{a \in V} {}^2D^3_{a,w} Y^3_{a,\gamma} Y^{3,*}_{a,\delta} \quad (3r_D r_T^2 N_v) \quad (6711)$$

$$\tau^1_{\gamma,\delta,w} = \sum_{i \in O} {}^2D^4_{i,w} Y^4_{i,\gamma} Y^{4,*}_{i,\delta} \quad (3r_D r_T^2 N_o) \quad (6712)$$

$$\tau^2_{\gamma,\delta,w} = \sum_{a \in V} {}^2D^1_{a,w} Y^1_{a,\gamma} Y^{1,*}_{a,\delta} \quad (3r_D r_T^2 N_v) \quad (6713)$$

$$\tau^3_{\alpha,i} = \sum_{a \in V} {}^1T_{a,i} W^4_{a,\alpha} \quad (2r_V N_o N_v) \quad (6714)$$

$$\tau^4_{\alpha,\beta} = \sum_{i \in O} W^1_{i,\alpha} \tau^3_{\beta,i} \quad (2r_V^2 N_o) \quad (6715)$$

$$\tau^5_{\alpha,i} = \sum_{\beta \in B} X_{\alpha,\beta} W^3_{i,\beta} \tau^4_{\alpha,\beta} \quad (3r_V^2 N_o) \quad (6716)$$

$$\tau^6_{i,j} = \sum_{\alpha \in B} W^2_{i,\alpha} \tau^5_{\alpha,j} \quad (2r_V N_o^2) \quad (6717)$$

$$\tau^7_{\gamma,i} = \sum_{j \in O} Y^2_{j,\gamma} \tau^6_{i,j} \quad (2r_T N_o^2) \quad (6718)$$

$$\tau^8_{\gamma,\delta,w} = \sum_{i \in O} {}^2D^2_{i,w} Y^{2,*}_{i,\delta} \tau^7_{\gamma,i} \quad (3r_D r_T^2 N_o) \quad (6719)$$

$$\tau^9_{\gamma,\delta,w} = \sum_{\epsilon \in A} Z_{\epsilon,\gamma} \tau^2_{\epsilon,\delta,w} \tau^8_{\epsilon,\delta,w} \quad (3r_D r_T^3) \quad (6720)$$

$${}^2R^z_{\gamma,\delta} \leftarrow \sum_{\epsilon \in A} \sum_{w \in D} \frac{1}{2} \tau^0_{\epsilon,\delta,w} \tau^1_{\epsilon,\delta,w} \tau^9_{\epsilon,\gamma,w} \quad (3r_D r_T^3) \quad (6721)$$

Raw expression

$${}^2R^z_{\epsilon,\zeta} \leftarrow \sum_{i \in O} \sum_{j \in O} \sum_{k \in O} \sum_{l \in O} \sum_{a \in V} \sum_{b \in V} \sum_{c \in V} \frac{1}{2} {}^1T_{c,k} Y^{1,*}_{a,\epsilon} Y^{2,*}_{i,\epsilon} Y^{3,*}_{b,\zeta} Y^{4,*}_{j,\zeta} {}^2D^{a,i,b,j} {}^2T_{a,l,b,j} V_{k,i,l,c} \quad (6722)$$

Factorized expression

$$\tau^0_{\gamma,\delta,w} = \sum_{a \in V} {}^2D^3_{a,w} Y^1_{a,\gamma} Y^{3,*}_{a,\delta} \quad (3r_D r_T^2 N_v) \quad (6723)$$



$$\tau^1_{\gamma,\delta,w} = \sum_{i \in O} {}^2D^4_{i,w} Y^2_{i,\gamma} Y^{4,*}_{i,\delta} \quad (3r_D r_T^2 N_o) \quad (6724)$$

$$\tau^2_{\gamma,\delta,w} = \sum_{\epsilon \in A} Z_{\epsilon,\gamma} \tau^0_{\epsilon,\delta,w} \tau^1_{\epsilon,\delta,w} \quad (3r_D r_T^3) \quad (6725)$$

$$\tau^3_{\gamma,\delta,w} = \sum_{a \in V} {}^2D^1_{a,w} Y^3_{a,\gamma} Y^{1,*}_{a,\delta} \quad (3r_D r_T^2 N_v) \quad (6726)$$

$$\tau^4_{\alpha,i} = \sum_{a \in V} {}^1T_{a,i} W^4_{a,\alpha} \quad (2r_V N_o N_v) \quad (6727)$$

$$\tau^5_{\alpha,\beta} = \sum_{i \in O} W^1_{i,\alpha} \tau^4_{\beta,i} \quad (2r_V^2 N_o) \quad (6728)$$

$$\tau^6_{\alpha,i} = \sum_{\beta \in B} X_{\alpha,\beta} W^3_{i,\beta} \tau^5_{\alpha,\beta} \quad (3r_V^2 N_o) \quad (6729)$$

$$\tau^7_{i,j} = \sum_{\alpha \in B} W^2_{i,\alpha} \tau^6_{\alpha,j} \quad (2r_V N_o^2) \quad (6730)$$

$$\tau^8_{\gamma,i} = \sum_{j \in O} Y^4_{j,\gamma} \tau^7_{i,j} \quad (2r_T N_o^2) \quad (6731)$$

$$\tau^9_{\gamma,\delta,w} = \sum_{i \in O} {}^2D^2_{i,w} Y^{2,*}_{i,\delta} \tau^8_{\gamma,i} \quad (3r_D r_T^2 N_o) \quad (6732)$$

$${}^2R^z_{\gamma,\delta} \leftarrow \sum_{\epsilon \in A} \sum_{w \in D} \frac{1}{2} \tau^2_{\epsilon,\delta,w} \tau^3_{\epsilon,\gamma,w} \tau^9_{\epsilon,\gamma,w} \quad (3r_D r_T^3) \quad (6733)$$

Raw expression

$${}^2R^z_{\epsilon,\zeta} \leftarrow \sum_{i \in O} \sum_{j \in O} \sum_{k \in O} \sum_{l \in O} \sum_{a \in V} \sum_{b \in V} \sum_{c \in V} \frac{1}{2} {}^1T_{c,k} Y^{1,*}_{a,\epsilon} Y^{2,*}_{i,\epsilon} Y^{3,*}_{b,\zeta} Y^{4,*}_{j,\zeta} {}^2D^{a,i,b,j} {}^2T_{b,j,a,l} V_{k,i,l,c} \quad (6734)$$

Factorized expression

$$\tau^0_{\gamma,\delta,w} = \sum_{a \in V} {}^2D^3_{a,w} Y^3_{a,\gamma} Y^{3,*}_{a,\delta} \quad (3r_D r_T^2 N_v) \quad (6735)$$

$$\tau^1_{\alpha,i} = \sum_{a \in V} {}^1T_{a,i} W^2_{a,\alpha} \quad (2r_V N_o N_v) \quad (6736)$$

$$\tau^2_{\alpha,\beta} = \sum_{i \in O} W^3_{i,\beta} \tau^1_{\alpha,i} \quad (2r_V^2 N_o) \quad (6737)$$

$$\tau^3_{\alpha,i} = \sum_{\beta \in B} X_{\alpha,\beta} W^4_{i,\beta} \tau^2_{\alpha,\beta} \quad (3r_V^2 N_o) \quad (6738)$$

$$\tau^4_{i,j} = \sum_{\alpha \in B} W^1_{i,\alpha} \tau^3_{\alpha,j} \quad (2r_V N_o^2) \quad (6739)$$

$$\tau^5_{\gamma,i} = \sum_{j \in O} Y^4_{j,\gamma} \tau^4_{j,i} \quad (2r_T N_o^2) \quad (6740)$$

$$\tau^6_{\gamma,\delta,w} = \sum_{i \in O} {}^2D^4_{i,w} Y^{4,*}_{i,\delta} \tau^5_{\gamma,i} \quad (3r_D r_T^2 N_o) \quad (6741)$$

$$\tau^7_{\gamma,\delta,w} = \sum_{a \in V} {}^2D^1_{a,w} Y^1_{a,\gamma} Y^{1,*}_{a,\delta} \quad (3r_D r_T^2 N_v) \quad (6742)$$

$$\tau^8_{\gamma,\delta,w} = \sum_{i \in O} {}^2D^2_{i,w} Y^2_{i,\gamma} Y^{2,*}_{i,\delta} \quad (3r_D r_T^2 N_o) \quad (6743)$$

$$\tau^9_{\gamma,\delta,w} = \sum_{\epsilon \in A} Z_{\epsilon,\gamma} \tau^7_{\epsilon,\delta,w} \tau^8_{\epsilon,\delta,w} \quad (3r_D r_T^3) \quad (6744)$$

$${}^2R^z_{\gamma,\delta} \leftarrow \sum_{\epsilon \in A} \sum_{w \in D} \frac{1}{2} \tau^0_{\epsilon,\delta,w} \tau^6_{\epsilon,\delta,w} \tau^9_{\epsilon,\gamma,w} \quad (3r_D r_T^3) \quad (6745)$$

Raw expression

$${}^2R^z_{\epsilon,\zeta} \leftarrow \sum_{i \in O} \sum_{j \in O} \sum_{k \in O} \sum_{l \in O} \sum_{a \in V} \sum_{b \in V} \sum_{c \in V} \frac{1}{2} {}^1T_{c,k} Y^{1,*}_{a,\epsilon} Y^{2,*}_{i,\epsilon} Y^{3,*}_{b,\zeta} Y^{4,*}_{j,\zeta} {}^2D^{a,i,b,j} {}^2T_{b,l,a,i} V_{l,c,k,j} \quad (6746)$$

Factorized expression

$$\tau^0_{\gamma,\delta,w} = \sum_{a \in V} {}^2D^3_{a,w} Y^1_{a,\gamma} Y^{3,*}_{a,\delta} \quad (3r_D r_T^2 N_v) \quad (6747)$$

$$\tau^1_{\alpha,i} = \sum_{a \in V} {}^1T_{a,i} W^2_{a,\alpha} \quad (2r_V N_o N_v) \quad (6748)$$

$$\tau^2_{\alpha,\beta} = \sum_{i \in O} W^3_{i,\beta} \tau^1_{\alpha,i} \quad (2r_V^2 N_o) \quad (6749)$$

$$\tau^3_{\alpha,i} = \sum_{\beta \in B} X_{\alpha,\beta} W^4_{i,\beta} \tau^2_{\alpha,\beta} \quad (3r_V^2 N_o) \quad (6750)$$

$$\tau^4_{i,j} = \sum_{\alpha \in B} W^1_{i,\alpha} \tau^3_{\alpha,j} \quad (2r_V N_o^2) \quad (6751)$$

$$\tau^5_{\gamma,i} = \sum_{j \in O} Y^2_{j,\gamma} \tau^4_{j,i} \quad (2r_T N_o^2) \quad (6752)$$

$$\tau^6_{\gamma,\delta,w} = \sum_{i \in O} {}^2D^4_{i,w} Y^{4,*}_{i,\delta} \tau^5_{\gamma,i} \quad (3r_D r_T^2 N_o) \quad (6753)$$

$$\tau^7_{\gamma,\delta,w} = \sum_{\epsilon \in A} Z_{\epsilon,\gamma} \tau^0_{\epsilon,\delta,w} \tau^6_{\epsilon,\delta,w} \quad (3r_D r_T^3) \quad (6754)$$

$$\tau^8_{\gamma,\delta,w} = \sum_{a \in V} {}^2D^1_{a,w} Y^3_{a,\gamma} Y^{1,*}_{a,\delta} \quad (3r_D r_T^2 N_v) \quad (6755)$$

$$\tau^9_{\gamma,\delta,w} = \sum_{i \in O} {}^2D^2_{i,w} Y^4_{i,\gamma} Y^{2,*}_{i,\delta} \quad (3r_D r_T^2 N_o) \quad (6756)$$

$${}^2R^z_{\gamma,\delta} \leftarrow \sum_{\epsilon \in A} \sum_{w \in D} \frac{1}{2} \tau^7_{\epsilon,\delta,w} \tau^8_{\epsilon,\gamma,w} \tau^9_{\epsilon,\gamma,w} \quad (3r_D r_T^3) \quad (6757)$$

Raw expression

$${}^2R^z_{\epsilon,\zeta} \leftarrow - \sum_{i \in O} \sum_{j \in O} \sum_{k \in O} \sum_{l \in O} \sum_{a \in V} \sum_{b \in V} \sum_{c \in V} {}^1T_{a,k} Y^{1,*}_{a,\epsilon} Y^{2,*}_{i,\epsilon} Y^{3,*}_{b,\zeta} Y^{4,*}_{j,\zeta} {}^2D^{a,i,b,j} {}^2T_{b,j,c,l} V_{k,i,l,c} \quad (6758)$$

Factorized expression

$$\tau^0_{\gamma,\delta,w} = \sum_{a \in V} {}^2D^3_{a,w} Y^1_{a,\gamma} Y^{3,*}_{a,\delta} \quad (3r_D r_T^2 N_v) \quad (6759)$$

$$\tau^1_{\gamma,\delta,w} = \sum_{i \in O} {}^2D^4_{i,w} Y^2_{i,\gamma} Y^{4,*}_{i,\delta} \quad (3r_D r_T^2 N_o) \quad (6760)$$

$$\tau^2_{\gamma,\delta,w} = \sum_{\epsilon \in A} Z_{\epsilon,\gamma} \tau^0_{\epsilon,\delta,w} \tau^1_{\epsilon,\delta,w} \quad (3r_D r_T^3) \quad (6761)$$

$$\tau^3_{\gamma,\delta,w} = \sum_{i \in O} {}^2D^2_{i,w} Y^4_{i,\gamma} Y^{2,*}_{i,\delta} \quad (3r_D r_T^2 N_o) \quad (6762)$$

$$\tau^4_{\gamma,w,i} = \sum_{a \in V} {}^2D^1_{a,w} {}^1T_{a,i} Y^{1,*}_{a,\gamma} \quad (3r_D r_T N_o N_v) \quad (6763)$$

$$\tau^5_{\gamma,i} = \sum_{a \in V} Y^3_{a,\gamma} f_{i,a} \quad (2r_T N_o N_v) \quad (6764)$$

$$\tau^6_{\gamma,\delta,w} = \sum_{i \in O} \tau^5_{\gamma,i} \tau^4_{\delta,w,i} \quad (2r_D r_T^2 N_o) \quad (6765)$$

$${}^2R^z_{\gamma,\delta} \leftarrow - \sum_{\epsilon \in A} \sum_{w \in D} \frac{1}{2} \tau^2_{\epsilon,\delta,w} \tau^3_{\epsilon,\gamma,w} \tau^6_{\epsilon,\gamma,w} \quad (3r_D r_T^3) \quad (6766)$$

Raw expression

$${}^2R^z_{\epsilon,\zeta} \leftarrow - \sum_{i \in O} \sum_{j \in O} \sum_{k \in O} \sum_{l \in O} \sum_{a \in V} \sum_{b \in V} \sum_{c \in V} {}^1T_{a,k} Y^{1,*}_{a,\epsilon} Y^{2,*}_{i,\epsilon} Y^{3,*}_{b,\zeta} Y^{4,*}_{j,\zeta} {}^2D^{a,i,b,j} {}^2T_{c,l,b,j} V_{k,i,l,c} \quad (6767)$$

Factorized expression

$$\tau^0_{\gamma,\delta,w} = \sum_{a \in V} {}^2D^3_{a,w} Y^3_{a,\gamma} Y^{3,*}_{a,\delta} \quad (3r_D r_T^2 N_v) \quad (6768)$$

$$\tau^1_{\gamma,\delta,w} = \sum_{i \in O} {}^2D^4_{i,w} Y^4_{i,\gamma} Y^{4,*}_{i,\delta} \quad (3r_D r_T^2 N_o) \quad (6769)$$

$$\tau^2_{\gamma,\delta,w} = \sum_{i \in O} {}^2D^2_{i,w} Y^2_{i,\gamma} Y^{2,*}_{i,\delta} \quad (3r_D r_T^2 N_o) \quad (6770)$$

$$\tau^3_{\gamma,w,i} = \sum_{a \in V} {}^2D^1_{a,w} {}^1T_{a,i} Y^{1,*}_{a,\gamma} \quad (3r_D r_T N_o N_v) \quad (6771)$$

$$\tau^4_{\gamma,i} = \sum_{a \in V} Y^1_{a,\gamma} f_{i,a} \quad (2r_T N_o N_v) \quad (6772)$$

$$\tau^5_{\gamma,\delta,w} = \sum_{i \in O} \tau^4_{\gamma,i} \tau^3_{\delta,w,i} \quad (2r_D r_T^2 N_o) \quad (6773)$$

$$\tau^6_{\gamma,\delta,w} = \sum_{\epsilon \in A} Z_{\epsilon,\gamma} \tau^2_{\epsilon,\delta,w} \tau^5_{\epsilon,\delta,w} \quad (3r_D r_T^3) \quad (6774)$$

$${}^2R^z_{\gamma,\delta} \leftarrow - \sum_{\epsilon \in A} \sum_{w \in D} \frac{1}{2} \tau^0_{\epsilon,\delta,w} \tau^1_{\epsilon,\delta,w} \tau^6_{\epsilon,\gamma,w} \quad (3r_D r_T^3) \quad (6775)$$

Raw expression

$${}^2R^z_{\epsilon,\zeta} \leftarrow - \sum_{i \in O} \sum_{j \in O} \sum_{k \in O} \sum_{l \in O} \sum_{a \in V} \sum_{b \in V} \sum_{c \in V} {}^1T_{b,k} Y^{1,*}_{a,\epsilon} Y^{2,*}_{i,\epsilon} Y^{3,*}_{b,\zeta} Y^{4,*}_{j,\zeta} {}^2D^{a,i,b,j} {}^2T_{a,i,c,l} V_{l,c,k,j} \quad (6776)$$

Factorized expression

$$\tau^0_{\gamma,\delta,w} = \sum_{i \in O} {}^2D^4_{i,w} Y^4_{i,\gamma} Y^{4,*}_{i,\delta} \quad (3r_D r_T^2 N_o) \quad (6777)$$

$$\tau^1_{\gamma,w,i} = \sum_{a \in V} {}^2D^3_{a,w} {}^1T_{a,i} Y^{3,*}_{a,\gamma} \quad (3r_D r_T N_o N_v) \quad (6778)$$

$$\tau^2_{\gamma,i} = \sum_{a \in V} Y^3_{a,\gamma} f_{i,a} \quad (2r_T N_o N_v) \quad (6779)$$

$$\tau^3_{\gamma,\delta,w} = \sum_{i \in O} \tau^2_{\gamma,i} \tau^1_{\delta,w,i} \quad (2r_D r_T^2 N_o) \quad (6780)$$

$$\tau^4_{\gamma,\delta,w} = \sum_{a \in V} {}^2D^1_{a,w} Y^1_{a,\gamma} Y^{1,*}_{a,\delta} \quad (3r_D r_T^2 N_v) \quad (6781)$$

$$\tau^5_{\gamma,\delta,w} = \sum_{i \in O} {}^2D^2_{i,w} Y^2_{i,\gamma} Y^{2,*}_{i,\delta} \quad (3r_D r_T^2 N_o) \quad (6782)$$

$$\tau^6_{\gamma,\delta,w} = \sum_{\epsilon \in A} Z_{\epsilon,\gamma} \tau^4_{\epsilon,\delta,w} \tau^5_{\epsilon,\delta,w} \quad (3r_D r_T^3) \quad (6783)$$

$${}^2R^z_{\gamma,\delta} \leftarrow - \sum_{\epsilon \in A} \sum_{w \in D} \frac{1}{2} \tau^0_{\epsilon,\delta,w} \tau^3_{\epsilon,\delta,w} \tau^6_{\epsilon,\gamma,w} \quad (3r_D r_T^3) \quad (6784)$$

Raw expression

$${}^2R^z_{\epsilon,\zeta} \leftarrow - \sum_{i \in O} \sum_{j \in O} \sum_{k \in O} \sum_{l \in O} \sum_{a \in V} \sum_{b \in V} \sum_{c \in V} {}^1T_{b,k} Y^{1,*}_{a,\epsilon} Y^{2,*}_{i,\epsilon} Y^{3,*}_{b,\zeta} Y^{4,*}_{j,\zeta} {}^2D^{a,i,b,j} {}^2T_{c,l,a,i} V_{l,c,k,j} \quad (6785)$$

Factorized expression

$$\tau^0_{\gamma,\delta,w} = \sum_{i \in O} {}^2D^4_{i,w} Y^2_{i,\gamma} Y^{4,*}_{i,\delta} \quad (3r_D r_T^2 N_o) \quad (6786)$$

$$\tau^1_{\gamma,w,i} = \sum_{a \in V} {}^2D^3_{a,w} {}^1T_{a,i} Y^{3,*}_{a,\gamma} \quad (3r_D r_T N_o N_v) \quad (6787)$$

$$\tau^2_{\gamma,i} = \sum_{a \in V} Y^1_{a,\gamma} f_{i,a} \quad (2r_T N_o N_v) \quad (6788)$$

$$\tau^3_{\gamma,\delta,w} = \sum_{i \in O} \tau^2_{\gamma,i} \tau^1_{\delta,w,i} \quad (2r_D r_T^2 N_o) \quad (6789)$$

$$\tau^4_{\gamma,\delta,w} = \sum_{\epsilon \in A} Z_{\epsilon,\gamma} \tau^0_{\epsilon,\delta,w} \tau^3_{\epsilon,\delta,w} \quad (3r_D r_T^3) \quad (6790)$$

$$\tau^5_{\gamma,\delta,w} = \sum_{a \in V} {}^2D^1_{a,w} Y^3_{a,\gamma} Y^{1,*}_{a,\delta} \quad (3r_D r_T^2 N_v) \quad (6791)$$

$$\tau^6_{\gamma,\delta,w} = \sum_{i \in O} {}^2D^2_{i,w} Y^4_{i,\gamma} Y^{2,*}_{i,\delta} \quad (3r_D r_T^2 N_o) \quad (6792)$$

$${}^2R^z_{\gamma,\delta} \leftarrow - \sum_{\epsilon \in A} \sum_{w \in D} \frac{1}{2} \tau^4_{\epsilon,\delta,w} \tau^5_{\epsilon,\gamma,w} \tau^6_{\epsilon,\gamma,w} \quad (3r_D r_T^3) \quad (6793)$$

Raw expression

$${}^2R^z_{\epsilon,\zeta} \leftarrow - \sum_{i \in O} \sum_{j \in O} \sum_{k \in O} \sum_{l \in O} \sum_{a \in V} \sum_{b \in V} \sum_{c \in V} {}^1T_{c,k} Y^{1,*}_{a,\epsilon} Y^{2,*}_{i,\epsilon} Y^{3,*}_{b,\zeta} Y^{4,*}_{j,\zeta} {}^2D^{a,i,b,j} {}^2T_{a,i,b,l} V_{k,c,l,j} \quad (6794)$$

Factorized expression

$$\tau^0_{\gamma,\delta,w} = \sum_{a \in V} {}^2D^3_{a,w} Y^3_{a,\gamma} Y^{3,*}_{a,\delta} \quad (3r_D r_T^2 N_v) \quad (6795)$$

$$\tau^1_{\gamma,\delta,w} = \sum_{i \in O} {}^2D^4_{i,w} Y^4_{i,\gamma} Y^{4,*}_{i,\delta} \quad (3r_D r_T^2 N_o) \quad (6796)$$

$$\tau^2_{\gamma,\delta,w} = \sum_{a \in V} {}^2D^1_{a,w} Y^1_{a,\gamma} Y^{1,*}_{a,\delta} \quad (3r_D r_T^2 N_v) \quad (6797)$$

$$\tau^3_{i,j} = \sum_{a \in V} {}^1T_{a,i} f_{j,a} \quad (2N_o^2 N_v) \quad (6798)$$

$$\tau^4_{\gamma,i} = \sum_{j \in O} Y^2_{j,\gamma} \tau^3_{i,j} \quad (2r_T N_o^2) \quad (6799)$$

$$\tau^5_{\gamma,\delta,w} = \sum_{i \in O} {}^2D^2_{i,w} Y^{2,*}_{i,\delta} \tau^4_{\gamma,i} \quad (3r_D r_T^2 N_o) \quad (6800)$$

$$\tau_{\gamma,\delta,w}^6 = \sum_{\epsilon \in A} Z_{\epsilon,\gamma} \tau_{\epsilon,\delta,w}^2 \tau_{\epsilon,\delta,w}^5 \quad (3r_D r_T^3) \quad (6801)$$

$${}^2R_{\gamma,\delta}^z \leftarrow - \sum_{\epsilon \in A} \sum_{w \in D} \frac{1}{2} \tau_{\epsilon,\delta,w}^0 \tau_{\epsilon,\delta,w}^1 \tau_{\epsilon,\gamma,w}^6 \quad (3r_D r_T^3) \quad (6802)$$

Raw expression

$${}^2R_{\epsilon,\zeta}^z \leftarrow - \sum_{i \in O} \sum_{j \in O} \sum_{k \in O} \sum_{l \in O} \sum_{a \in V} \sum_{b \in V} \sum_{c \in V} {}^1T_{c,k} Y^{1,*}_{a,\epsilon} Y^{2,*}_{i,\epsilon} Y^{3,*}_{b,\zeta} Y^{4,*}_{j,\zeta} {}^2D^{a,i,b,j} {}^2T_{a,l,b,j} V_{l,i,k,c} \quad (6803)$$

Factorized expression

$$\tau_{\gamma,\delta,w}^0 = \sum_{a \in V} {}^2D^3_{a,w} Y^1_{a,\gamma} Y^{3,*}_{a,\delta} \quad (3r_D r_T^2 N_v) \quad (6804)$$

$$\tau_{\gamma,\delta,w}^1 = \sum_{i \in O} {}^2D^4_{i,w} Y^2_{i,\gamma} Y^{4,*}_{i,\delta} \quad (3r_D r_T^2 N_o) \quad (6805)$$

$$\tau_{\gamma,\delta,w}^2 = \sum_{\epsilon \in A} Z_{\epsilon,\gamma} \tau_{\epsilon,\delta,w}^0 \tau_{\epsilon,\delta,w}^1 \quad (3r_D r_T^3) \quad (6806)$$

$$\tau_{\gamma,\delta,w}^3 = \sum_{a \in V} {}^2D^1_{a,w} Y^3_{a,\gamma} Y^{1,*}_{a,\delta} \quad (3r_D r_T^2 N_v) \quad (6807)$$

$$\tau_{i,j}^4 = \sum_{a \in V} {}^1T_{a,i} f_{j,a} \quad (2N_o^2 N_v) \quad (6808)$$

$$\tau_{\gamma,i}^5 = \sum_{j \in O} Y^4_{j,\gamma} \tau_{i,j}^4 \quad (2r_T N_o^2) \quad (6809)$$

$$\tau_{\gamma,\delta,w}^6 = \sum_{i \in O} {}^2D^2_{i,w} Y^{2,*}_{i,\delta} \tau_{\gamma,i}^5 \quad (3r_D r_T^2 N_o) \quad (6810)$$

$${}^2R_{\gamma,\delta}^z \leftarrow - \sum_{\epsilon \in A} \sum_{w \in D} \frac{1}{2} \tau_{\epsilon,\delta,w}^2 \tau_{\epsilon,\gamma,w}^3 \tau_{\epsilon,\gamma,w}^6 \quad (3r_D r_T^3) \quad (6811)$$

Raw expression

$${}^2R_{\epsilon,\zeta}^z \leftarrow - \sum_{i \in O} \sum_{j \in O} \sum_{k \in O} \sum_{l \in O} \sum_{a \in V} \sum_{b \in V} \sum_{c \in V} {}^1T_{c,k} Y^{1,*}_{a,\epsilon} Y^{2,*}_{i,\epsilon} Y^{3,*}_{b,\zeta} Y^{4,*}_{j,\zeta} {}^2D^{a,i,b,j} {}^2T_{b,j,a,l} V_{l,i,k,c} \quad (6812)$$

Factorized expression

$$\tau_{\gamma,\delta,w}^0 = \sum_{a \in V} {}^2D^3_{a,w} Y^3_{a,\gamma} Y^{3,*}_{a,\delta} \quad (3r_D r_T^2 N_v) \quad (6813)$$

$$\tau_{i,j}^1 = \sum_{a \in V} {}^1T_{a,i} f_{j,a} \quad (2N_o^2 N_v) \quad (6814)$$

$$\tau_{\gamma,i}^2 = \sum_{j \in O} Y^4_{j,\gamma} \tau_{i,j}^1 \quad (2r_T N_o^2) \quad (6815)$$

$$\tau_{\gamma,\delta,w}^3 = \sum_{i \in O} {}^2D^4_{i,w} Y^{4,*}_{i,\delta} \tau_{\gamma,i}^2 \quad (3r_D r_T^2 N_o) \quad (6816)$$

$$\tau_{\gamma,\delta,w}^4 = \sum_{a \in V} {}^2D^1_{a,w} Y^1_{a,\gamma} Y^{1,*}_{a,\delta} \quad (3r_D r_T^2 N_v) \quad (6817)$$

$$\tau_{\gamma,\delta,w}^5 = \sum_{i \in O} {}^2D^2_{i,w} Y^2_{i,\gamma} Y^{2,*}_{i,\delta} \quad (3r_D r_T^2 N_o) \quad (6818)$$

$$\tau_{\gamma,\delta,w}^6 = \sum_{\epsilon \in A} Z_{\epsilon,\gamma} \tau_{\epsilon,\delta,w}^4 \tau_{\epsilon,\delta,w}^5 \quad (3r_D r_T^3) \quad (6819)$$

$${}^2R_{\gamma,\delta}^z \leftarrow - \sum_{\epsilon \in A} \sum_{w \in D} \frac{1}{2} \tau_{\epsilon,\delta,w}^0 \tau_{\epsilon,\delta,w}^3 \tau_{\epsilon,\gamma,w}^6 \quad (3r_D r_T^3) \quad (6820)$$

Raw expression

$${}^2R_{\epsilon,\zeta}^z \leftarrow - \sum_{i \in O} \sum_{j \in O} \sum_{k \in O} \sum_{l \in O} \sum_{a \in V} \sum_{b \in V} \sum_{c \in V} {}^1T_{c,k} Y^{1,*}_{a,\epsilon} Y^{2,*}_{i,\epsilon} Y^{3,*}_{b,\zeta} Y^{4,*}_{j,\zeta} {}^2D^{a,i,b,j} {}^2T_{b,l,a,i} V_{k,c,l,j} \quad (6821)$$

Factorized expression

$$\tau_{\gamma,\delta,w}^0 = \sum_{a \in V} {}^2D^3_{a,w} Y^1_{a,\gamma} Y^{3,*}_{a,\delta} \quad (3r_D r_T^2 N_v) \quad (6822)$$

$$\tau_{i,j}^1 = \sum_{a \in V} {}^1T_{a,i} f_{j,a} \quad (2N_o^2 N_v) \quad (6823)$$

$$\tau_{\gamma,i}^2 = \sum_{j \in O} Y^2_{j,\gamma} \tau_{i,j}^1 \quad (2r_T N_o^2) \quad (6824)$$

$$\tau_{\gamma,\delta,w}^3 = \sum_{i \in O} {}^2D^4_{i,w} Y^{4,*}_{i,\delta} \tau_{\gamma,i}^2 \quad (3r_D r_T^2 N_o) \quad (6825)$$

$$\tau^4_{\gamma,\delta,w} = \sum_{\epsilon \in A} Z_{\epsilon,\gamma} \tau^0_{\epsilon,\delta,w} \tau^3_{\epsilon,\delta,w} \quad (3r_D r_T^3) \quad (6826)$$

$$\tau^5_{\gamma,\delta,w} = \sum_{a \in V} {}^2D^1_{a,w} Y^3_{a,\gamma} Y^{1,*}_{a,\delta} \quad (3r_D r_T^2 N_v) \quad (6827)$$

$$\tau^6_{\gamma,\delta,w} = \sum_{i \in O} {}^2D^2_{i,w} Y^4_{i,\gamma} Y^{2,*}_{i,\delta} \quad (3r_D r_T^2 N_o) \quad (6828)$$

$${}^2R^z_{\gamma,\delta} \leftarrow - \sum_{\epsilon \in A} \sum_{w \in D} \frac{1}{2} \tau^4_{\epsilon,\delta,w} \tau^5_{\epsilon,\gamma,w} \tau^6_{\epsilon,\gamma,w} \quad (3r_D r_T^3) \quad (6829)$$

### G. Contributions from $(H^1 T^1 T^1 T^1 T)_c$

Raw expression

$${}^2R^z_{\epsilon,\zeta} \leftarrow \sum_{i \in O} \sum_{j \in O} \sum_{k \in O} \sum_{l \in O} \sum_{a \in V} \sum_{b \in V} \sum_{c \in V} \sum_{d \in V} {}^1T_{a,k} {}^1T_{b,l} {}^1T_{c,i} {}^1T_{d,j} Y^{1,*}_{a,\epsilon} Y^{2,*}_{i,\epsilon} Y^{3,*}_{b,\zeta} Y^{4,*}_{j,\zeta} {}^2D^{a,i,b,j}_{k,c,l,d} V_{k,c,l,d} \quad (6830)$$

Factorized expression

$$\tau^0_{\alpha,i} = \sum_{a \in V} {}^1T_{a,i} W^4_{a,\alpha} \quad (2r_V N_o N_v) \quad (6831)$$

$$\tau^1_{\gamma,\alpha,w} = \sum_{i \in O} {}^2D^4_{i,w} Y^{4,*}_{i,\gamma} \tau^0_{\alpha,i} \quad (3r_D r_T r_V N_o) \quad (6832)$$

$$\tau^2_{\gamma,w,i} = \sum_{a \in V} {}^2D^3_{a,w} {}^1T_{a,i} Y^{3,*}_{a,\gamma} \quad (3r_D r_T N_o N_v) \quad (6833)$$

$$\tau^3_{\gamma,\alpha,w} = \sum_{i \in O} W^3_{i,\alpha} \tau^2_{\gamma,w,i} \quad (2r_D r_T r_V N_o) \quad (6834)$$

$$\tau^4_{\gamma,\alpha,w} = \sum_{\beta \in B} X_{\alpha,\beta} \tau^1_{\gamma,\beta,w} \tau^3_{\gamma,\beta,w} \quad (3r_D r_T r_V^2) \quad (6835)$$

$$\tau^5_{\alpha,i} = \sum_{a \in V} {}^1T_{a,i} W^2_{a,\alpha} \quad (2r_V N_o N_v) \quad (6836)$$

$$\tau^6_{\gamma,\alpha,w} = \sum_{i \in O} {}^2D^2_{i,w} Y^{2,*}_{i,\gamma} \tau^5_{\alpha,i} \quad (3r_D r_T r_V N_o) \quad (6837)$$

$$\tau^7_{\gamma,w,i} = \sum_{a \in V} {}^2D^1_{a,w} {}^1T_{a,i} Y^{1,*}_{a,\gamma} \quad (3r_D r_T N_o N_v) \quad (6838)$$

$$\tau^8_{\gamma,\alpha,w} = \sum_{i \in O} W^1_{i,\alpha} \tau^7_{\gamma,w,i} \quad (2r_D r_T r_V N_o) \quad (6839)$$

$${}^2R^z_{\gamma,\delta} \leftarrow \sum_{\alpha \in B} \sum_{w \in D} \tau^4_{\delta,\alpha,w} \tau^6_{\gamma,\alpha,w} \tau^8_{\gamma,\alpha,w} \quad (3r_D r_T^2 r_V) \quad (6840)$$

### H. Contributions from $(H^1 T^1 T^2 T)_c$

Raw expression

$${}^2R^z_{\epsilon,\zeta} \leftarrow \sum_{i \in O} \sum_{j \in O} \sum_{k \in O} \sum_{l \in O} \sum_{a \in V} \sum_{b \in V} \sum_{c \in V} \sum_{d \in V} \frac{1}{2} {}^1T_{a,k} {}^1T_{b,l} Y^{1,*}_{a,\epsilon} Y^{2,*}_{i,\epsilon} Y^{3,*}_{b,\zeta} Y^{4,*}_{j,\zeta} {}^2D^{a,i,b,j}_{c,i,d,j} V_{k,c,l,d} \quad (6841)$$

Factorized expression

$$\tau^0_{\gamma,\delta,w} = \sum_{a \in V} {}^2D^3_{a,w} Y^1_{a,\gamma} Y^{3,*}_{a,\delta} \quad (3r_D r_T^2 N_v) \quad (6842)$$

$$\tau^1_{\gamma,\delta,w} = \sum_{i \in O} {}^2D^4_{i,w} Y^2_{i,\gamma} Y^{4,*}_{i,\delta} \quad (3r_D r_T^2 N_o) \quad (6843)$$

$$\tau^2_{\alpha,i} = \sum_{a \in V} {}^1T_{a,i} W^2_{a,\alpha} \quad (2r_V N_o N_v) \quad (6844)$$

$$\tau^3_{\gamma,\alpha,w} = \sum_{i \in O} {}^2D^2_{i,w} Y^{2,*}_{i,\gamma} \tau^2_{\alpha,i} \quad (3r_D r_T r_V N_o) \quad (6845)$$

$$\tau^4_{\gamma,w,i} = \sum_{a \in V} {}^2D^1_{a,w} {}^1T_{a,i} Y^{1,*}_{a,\gamma} \quad (3r_D r_T N_o N_v) \quad (6846)$$

$$\tau^5_{\gamma,\alpha,w} = \sum_{i \in O} W^1_{i,\alpha} \tau^4_{\gamma,w,i} \quad (2r_D r_T r_V N_o) \quad (6847)$$

$$\tau^6_{\gamma,\alpha} = \sum_{a \in V} W^4_{a,\alpha} Y^3_{a,\gamma} \quad (2r_T r_V N_v) \quad (6848)$$

$$\tau^7_{\gamma,\alpha} = \sum_{i \in O} W^3_{i,\alpha} Y^4_{i,\gamma} \quad (2r_T r_V N_o) \quad (6849)$$

$$\tau^8_{\gamma,\alpha} = \sum_{\beta \in B} X_{\alpha,\beta} \tau^6_{\gamma,\beta} \tau^7_{\gamma,\beta} \quad (3r_T r_V^2) \quad (6850)$$

$$\tau^8_{\gamma,\alpha} = \sum_{\beta \in B} X_{\alpha,\beta} \tau^6_{\gamma,\beta} \tau^7_{\gamma,\beta} \quad (3r_T r_V^2) \quad (6863)$$

$$\tau^9_{\gamma,\alpha} = \sum_{\delta \in A} Z_{\gamma,\delta} \tau^8_{\delta,\alpha} \quad (2r_T^2 r_V) \quad (6851)$$

$$\tau^9_{\gamma,\alpha} = \sum_{\delta \in A} Z_{\delta,\gamma} \tau^8_{\delta,\alpha} \quad (2r_T^2 r_V) \quad (6864)$$

$$\tau^{10}_{\gamma,\delta,w} = \sum_{\alpha \in B} \tau^9_{\gamma,\alpha} \tau^3_{\delta,\alpha,w} \tau^5_{\delta,\alpha,w} \quad (3r_D r_T^2 r_V) \quad (6852)$$

$$\tau^{10}_{\gamma,\delta,w} = \sum_{\alpha \in B} \tau^9_{\gamma,\alpha} \tau^3_{\delta,\alpha,w} \tau^5_{\delta,\alpha,w} \quad (3r_D r_T^2 r_V) \quad (6865)$$

$${}^2R^z_{\gamma,\delta} \leftarrow - \sum_{\epsilon \in A} \sum_{w \in D} \tau^0_{\epsilon,\delta,w} \tau^1_{\epsilon,\delta,w} \tau^{10}_{\epsilon,\gamma,w} \quad (3r_D r_T^3) \quad (6853)$$

$${}^2R^z_{\gamma,\delta} \leftarrow - \sum_{\epsilon \in A} \sum_{w \in D} \tau^0_{\epsilon,\delta,w} \tau^1_{\epsilon,\delta,w} \tau^{10}_{\epsilon,\gamma,w} \quad (3r_D r_T^3) \quad (6866)$$

Raw expression

$${}^2R^z_{\epsilon,\zeta} \leftarrow \sum_{i \in O} \sum_{j \in O} \sum_{k \in O} \sum_{l \in O} \sum_{a \in V} \sum_{b \in V} \sum_{c \in V} \sum_{d \in V} \frac{1}{2} \quad (6854)$$

$$\begin{aligned} & {}^1T_{a,k} \quad {}^1T_{b,l} \quad Y^{1,*}_{a,\epsilon} \quad Y^{2,*}_{i,\epsilon} \quad Y^{3,*}_{b,\zeta} \\ & Y^{4,*}_{j,\zeta} \quad {}^2D^{a,i,b,j} \quad {}^2T_{c,j,d,i} \quad V_{k,d,l,c} \end{aligned}$$

Raw expression

$${}^2R^z_{\epsilon,\zeta} \leftarrow \sum_{i \in O} \sum_{j \in O} \sum_{k \in O} \sum_{l \in O} \sum_{a \in V} \sum_{b \in V} \sum_{c \in V} \sum_{d \in V} \frac{1}{2} \quad (6867)$$

$$\begin{aligned} & {}^1T_{a,k} \quad {}^1T_{c,i} \quad Y^{1,*}_{a,\epsilon} \quad Y^{2,*}_{i,\epsilon} \quad Y^{3,*}_{b,\zeta} \\ & Y^{4,*}_{j,\zeta} \quad {}^2D^{a,i,b,j} \quad {}^2T_{b,j,d,l} \quad V_{k,d,l,c} \end{aligned}$$

Factorized expression

$$\tau^0_{\gamma,\delta,w} = \sum_{a \in V} {}^2D^3_{a,w} Y^3_{a,\gamma} Y^{3,*}_{a,\delta} \quad (3r_D r_T^2 N_v) \quad (6855)$$

$$\tau^0_{\gamma,\delta,w} = \sum_{i \in O} {}^2D^2_{i,w} Y^4_{i,\gamma} Y^{2,*}_{i,\delta} \quad (3r_D r_T^2 N_o) \quad (6868)$$

$$\tau^1_{\gamma,\delta,w} = \sum_{i \in O} {}^2D^4_{i,w} Y^4_{i,\gamma} Y^{4,*}_{i,\delta} \quad (3r_D r_T^2 N_o) \quad (6856)$$

$$\tau^1_{\gamma,w,i} = \sum_{a \in V} {}^2D^1_{a,w} {}^1T_{a,i} Y^{1,*}_{a,\gamma} \quad (3r_D r_T N_o N_v) \quad (6869)$$

$$\tau^2_{\alpha,i} = \sum_{a \in V} {}^1T_{a,i} W^2_{a,\alpha} \quad (2r_V N_o N_v) \quad (6857)$$

$$\tau^2_{\alpha,i} = \sum_{a \in V} {}^1T_{a,i} W^4_{a,\alpha} \quad (2r_V N_o N_v) \quad (6870)$$

$$\tau^3_{\gamma,\alpha,w} = \sum_{i \in O} {}^2D^2_{i,w} Y^{2,*}_{i,\gamma} \tau^2_{\alpha,i} \quad (3r_D r_T r_V N_o) \quad (6858)$$

$$\tau^3_{\alpha} = \sum_{i \in O} W^3_{i,\alpha} \tau^2_{\alpha,i} \quad (2r_V N_o) \quad (6871)$$

$$\tau^4_{\gamma,w,i} = \sum_{a \in V} {}^2D^1_{a,w} {}^1T_{a,i} Y^{1,*}_{a,\gamma} \quad (3r_D r_T N_o N_v) \quad (6859)$$

$$\tau^4_{\alpha} = \sum_{\beta \in B} \tau^3_{\beta} X_{\alpha,\beta} \quad (2r_V^2) \quad (6872)$$

$$\tau^5_{\gamma,\alpha,w} = \sum_{i \in O} W^1_{i,\alpha} \tau^4_{\gamma,w,i} \quad (2r_D r_T r_V N_o) \quad (6860)$$

$$\tau^5_{i,a} = \sum_{\alpha \in B} \tau^4_{\alpha} W^1_{i,\alpha} W^2_{a,\alpha} \quad (3r_V N_o N_v) \quad (6873)$$

$$\tau^6_{\gamma,\alpha} = \sum_{a \in V} W^4_{a,\alpha} Y^1_{a,\gamma} \quad (2r_T r_V N_v) \quad (6861)$$

$$\tau^6_{\gamma,i} = \sum_{a \in V} Y^3_{a,\gamma} \tau^5_{i,a} \quad (2r_T N_o N_v) \quad (6874)$$

$$\tau^7_{\gamma,\alpha} = \sum_{i \in O} W^3_{i,\alpha} Y^2_{i,\gamma} \quad (2r_T r_V N_o) \quad (6862)$$

$$\tau^7_{\gamma,\delta,w} = \sum_{i \in O} \tau^6_{\gamma,i} \tau^1_{\delta,w,i} \quad (2r_D r_T^2 N_o) \quad (6875)$$

$$\tau_{\gamma,\delta,w}^8 = \sum_{a \in V} {}^2D_{a,w}^3 Y_{a,\gamma}^1 Y_{a,\delta}^{3,*} \quad (3r_D r_T^2 N_v) \quad (6876)$$

$$\tau_{\gamma,\delta,w}^8 = \sum_{\epsilon \in A} Z_{\epsilon,\gamma} \tau_{\epsilon,\delta,w}^0 \tau_{\epsilon,\delta,w}^7 \quad (3r_D r_T^3) \quad (6889)$$

$$\tau_{\gamma,\delta,w}^9 = \sum_{i \in O} {}^2D_{i,w}^4 Y_{i,\gamma}^2 Y_{i,\delta}^{4,*} \quad (3r_D r_T^2 N_o) \quad (6877)$$

$$\tau_{\gamma,\delta,w}^9 = \sum_{a \in V} {}^2D_{a,w}^3 Y_{a,\gamma}^3 Y_{a,\delta}^{3,*} \quad (3r_D r_T^2 N_v) \quad (6890)$$

$$\tau_{\gamma,\delta,w}^{10} = \sum_{\epsilon \in A} Z_{\epsilon,\gamma} \tau_{\epsilon,\delta,w}^8 \tau_{\epsilon,\delta,w}^9 \quad (3r_D r_T^3) \quad (6878)$$

$$\tau_{\gamma,\delta,w}^{10} = \sum_{i \in O} {}^2D_{i,w}^4 Y_{i,\gamma}^4 Y_{i,\delta}^{4,*} \quad (3r_D r_T^2 N_o) \quad (6891)$$

$${}^2R_{\gamma,\delta}^z \leftarrow - \sum_{\epsilon \in A} \sum_{w \in D} \tau_{\epsilon,\gamma,w}^0 \tau_{\epsilon,\delta,w}^{10} \tau_{\epsilon,\gamma,w}^7 \quad (3r_D r_T^3) \quad (6879)$$

$${}^2R_{\gamma,\delta}^z \leftarrow - \sum_{\epsilon \in A} \sum_{w \in D} \tau_{\epsilon,\delta,w}^{10} \tau_{\epsilon,\gamma,w}^8 \tau_{\epsilon,\delta,w}^9 \quad (3r_D r_T^3) \quad (6892)$$

Raw expression

$${}^2R_{\epsilon,\zeta}^z \leftarrow \sum_{i \in O} \sum_{j \in O} \sum_{k \in O} \sum_{l \in O} \sum_{a \in V} \sum_{b \in V} \sum_{c \in V} \sum_{d \in V} \frac{1}{2} \quad (6880)$$

$$\begin{aligned} & {}^1T_{a,k} {}^1T_{c,i} Y_{a,\epsilon}^{1,*} Y_{i,\epsilon}^{2,*} Y_{b,\zeta}^{3,*} \\ & Y_{j,\zeta}^{4,*} {}^2D_{a,i,b,j} {}^2T_{b,l,d,j} V_{k,c,l,d} \end{aligned}$$

Raw expression

$${}^2R_{\epsilon,\zeta}^z \leftarrow \sum_{i \in O} \sum_{j \in O} \sum_{k \in O} \sum_{l \in O} \sum_{a \in V} \sum_{b \in V} \sum_{c \in V} \sum_{d \in V} \frac{1}{2} \quad (6893)$$

$$\begin{aligned} & {}^1T_{a,k} {}^1T_{c,i} Y_{a,\epsilon}^{1,*} Y_{i,\epsilon}^{2,*} Y_{b,\zeta}^{3,*} \\ & Y_{j,\zeta}^{4,*} {}^2D_{a,i,b,j} {}^2T_{d,j,b,l} V_{k,c,l,d} \end{aligned}$$

Factorized expression

$$\tau_{\gamma,\delta,w}^0 = \sum_{i \in O} {}^2D_{i,w}^2 Y_{i,\gamma}^2 Y_{i,\delta}^{2,*} \quad (3r_D r_T^2 N_o) \quad (6881)$$

$$\tau_{\alpha,i}^0 = \sum_{a \in V} {}^1T_{a,i} W_{a,\alpha}^2 \quad (2r_V N_o N_v) \quad (6894)$$

$$\tau_{\gamma,w,i}^1 = \sum_{a \in V} {}^2D_{a,w}^1 {}^1T_{a,i} Y_{a,\gamma}^{1,*} \quad (3r_D r_T N_o N_v) \quad (6882)$$

$$\tau_{\gamma,\alpha,w}^1 = \sum_{i \in O} {}^2D_{i,w}^4 Y_{i,\gamma}^{4,*} \tau_{\alpha,i}^0 \quad (3r_D r_T r_V N_o) \quad (6895)$$

$$\tau_{\alpha,i}^2 = \sum_{a \in V} {}^1T_{a,i} W_{a,\alpha}^4 \quad (2r_V N_o N_v) \quad (6883)$$

$$\tau_{\gamma,w,i}^2 = \sum_{a \in V} {}^2D_{a,w}^3 {}^1T_{a,i} Y_{a,\gamma}^{3,*} \quad (3r_D r_T N_o N_v) \quad (6896)$$

$$\tau_{\alpha}^3 = \sum_{i \in O} W_{i,\alpha}^3 \tau_{\alpha,i}^2 \quad (2r_V N_o) \quad (6884)$$

$$\tau_{\gamma,\alpha,w}^3 = \sum_{i \in O} W_{i,\alpha}^1 \tau_{\gamma,w,i}^2 \quad (2r_D r_T r_V N_o) \quad (6897)$$

$$\tau_{\alpha}^4 = \sum_{\beta \in B} \tau_{\beta}^3 X_{\alpha,\beta} \quad (2r_V^2) \quad (6885)$$

$$\tau_{\gamma,\alpha}^4 = \sum_{a \in V} W_{a,\alpha}^4 Y_{a,\gamma}^3 \quad (2r_T r_V N_v) \quad (6898)$$

$$\tau_{i,a}^5 = \sum_{\alpha \in B} \tau_{\alpha}^4 W_{i,\alpha}^1 W_{a,\alpha}^2 \quad (3r_V N_o N_v) \quad (6886)$$

$$\tau_{\gamma,\alpha}^5 = \sum_{i \in O} W_{i,\alpha}^3 Y_{i,\gamma}^4 \quad (2r_T r_V N_o) \quad (6899)$$

$$\tau_{\gamma,i}^6 = \sum_{a \in V} Y_{a,\gamma}^1 \tau_{i,a}^5 \quad (2r_T N_o N_v) \quad (6887)$$

$$\tau_{\gamma,\alpha}^6 = \sum_{\beta \in B} X_{\alpha,\beta} \tau_{\gamma,\beta}^4 \tau_{\gamma,\beta}^5 \quad (3r_T r_V^2) \quad (6900)$$

$$\tau_{\gamma,\delta,w}^7 = \sum_{i \in O} \tau_{\gamma,i}^6 \tau_{\delta,w,i}^1 \quad (2r_D r_T^2 N_o) \quad (6888)$$

$$\tau_{\gamma,\alpha}^7 = \sum_{\delta \in A} Z_{\gamma,\delta} \tau_{\delta,\alpha}^6 \quad (2r_T^2 r_V) \quad (6901)$$

$$\tau_{\gamma,\delta,w}^8 = \sum_{\alpha \in B} \tau_{\gamma,\alpha}^7 \tau_{\delta,\alpha,w}^1 \tau_{\delta,\alpha,w}^3 \quad (3r_D r_T^2 r_V) \quad (6902)$$

$$\tau_{\gamma,\delta,w}^8 = \sum_{\alpha \in B} \tau_{\gamma,\alpha}^7 \tau_{\delta,\alpha,w}^1 \tau_{\delta,\alpha,w}^3 \quad (3r_D r_T^2 r_V) \quad (6915)$$

$$\tau_{\gamma,\delta,w}^9 = \sum_{a \in V} {}^2D_{a,w}^1 Y_{a,\gamma}^1 Y_{a,\delta}^{1,*} \quad (3r_D r_T^2 N_v) \quad (6903)$$

$$\tau_{\gamma,\delta,w}^9 = \sum_{a \in V} {}^2D_{a,w}^1 Y_{a,\gamma}^3 Y_{a,\delta}^{1,*} \quad (3r_D r_T^2 N_v) \quad (6916)$$

$$\tau_{\gamma,\delta,w}^{10} = \sum_{i \in O} {}^2D_{i,w}^2 Y_{i,\gamma}^2 Y_{i,\delta}^{2,*} \quad (3r_D r_T^2 N_o) \quad (6904)$$

$$\tau_{\gamma,\delta,w}^{10} = \sum_{i \in O} {}^2D_{i,w}^2 Y_{i,\gamma}^4 Y_{i,\delta}^{2,*} \quad (3r_D r_T^2 N_o) \quad (6917)$$

$${}^2R_{\gamma,\delta}^z \leftarrow - \sum_{\epsilon \in A} \sum_{w \in D} \tau_{\epsilon,\gamma,w}^{10} \tau_{\epsilon,\delta,w}^8 \tau_{\epsilon,\gamma,w}^9 \quad (3r_D r_T^3) \quad (6905)$$

$${}^2R_{\gamma,\delta}^z \leftarrow - \sum_{\epsilon \in A} \sum_{w \in D} \tau_{\epsilon,\gamma,w}^{10} \tau_{\epsilon,\delta,w}^8 \tau_{\epsilon,\gamma,w}^9 \quad (3r_D r_T^3) \quad (6918)$$

Raw expression

Raw expression

$${}^2R_{\epsilon,\zeta}^z \leftarrow \sum_{i \in O} \sum_{j \in O} \sum_{k \in O} \sum_{l \in O} \sum_{a \in V} \sum_{b \in V} \sum_{c \in V} \sum_{d \in V} \frac{1}{2} \quad (6906)$$

$$\begin{aligned} & {}^1T_{a,k} {}^1T_{c,i} Y_{a,\epsilon}^{1,*} Y_{i,\epsilon}^{2,*} Y_{b,\zeta}^{3,*} \\ & Y_{j,\zeta}^{4,*} {}^2D_{a,i,b,j} {}^2T_{d,l,b,j} V_{k,d,l,c} \end{aligned}$$

$${}^2R_{\epsilon,\zeta}^z \leftarrow \sum_{i \in O} \sum_{j \in O} \sum_{k \in O} \sum_{l \in O} \sum_{a \in V} \sum_{b \in V} \sum_{c \in V} \sum_{d \in V} \frac{1}{2} \quad (6919)$$

$$\begin{aligned} & {}^1T_{a,k} {}^1T_{c,j} Y_{a,\epsilon}^{1,*} Y_{i,\epsilon}^{2,*} Y_{b,\zeta}^{3,*} \\ & Y_{j,\zeta}^{4,*} {}^2D_{a,i,b,j} {}^2T_{b,l,d,i} V_{k,d,l,c} \end{aligned}$$

Factorized expression

Factorized expression

$$\tau_{\alpha,i}^0 = \sum_{a \in V} {}^1T_{a,i} W_{a,\alpha}^2 \quad (2r_V N_o N_v) \quad (6907)$$

$$\tau_{\gamma,\delta,w}^0 = \sum_{a \in V} {}^2D_{a,w}^1 Y_{a,\gamma}^1 Y_{a,\delta}^{1,*} \quad (3r_D r_T^2 N_v) \quad (6920)$$

$$\tau_{\gamma,\alpha,w}^1 = \sum_{i \in O} {}^2D_{i,w}^4 Y_{i,\gamma}^{4,*} \tau_{\alpha,i}^0 \quad (3r_D r_T r_V N_o) \quad (6908)$$

$$\tau_{\gamma,\delta,w}^1 = \sum_{i \in O} {}^2D_{i,w}^2 Y_{i,\gamma}^2 Y_{i,\delta}^{2,*} \quad (3r_D r_T^2 N_o) \quad (6921)$$

$$\tau_{\gamma,w,i}^2 = \sum_{a \in V} {}^2D_{a,w}^3 {}^1T_{a,i} Y_{a,\gamma}^{3,*} \quad (3r_D r_T N_o N_v) \quad (6909)$$

$$\tau_{\gamma,\delta,w}^2 = \sum_{\epsilon \in A} Z_{\epsilon,\gamma} \tau_{\epsilon,\delta,w}^0 \tau_{\epsilon,\delta,w}^1 \quad (3r_D r_T^3) \quad (6922)$$

$$\tau_{\gamma,\alpha,w}^3 = \sum_{i \in O} W_{i,\alpha}^1 \tau_{\gamma,w,i}^2 \quad (2r_D r_T r_V N_o) \quad (6910)$$

$$\tau_{\gamma,\delta,w}^3 = \sum_{i \in O} {}^2D_{i,w}^4 Y_{i,\gamma}^4 Y_{i,\delta}^{4,*} \quad (3r_D r_T^2 N_o) \quad (6923)$$

$$\tau_{\gamma,\alpha}^4 = \sum_{a \in V} W_{a,\alpha}^4 Y_{a,\gamma}^1 \quad (2r_T r_V N_v) \quad (6911)$$

$$\tau_{\gamma,w,i}^4 = \sum_{a \in V} {}^2D_{a,w}^3 {}^1T_{a,i} Y_{a,\gamma}^{3,*} \quad (3r_D r_T N_o N_v) \quad (6924)$$

$$\tau_{\gamma,\alpha}^5 = \sum_{i \in O} W_{i,\alpha}^3 Y_{i,\gamma}^2 \quad (2r_T r_V N_o) \quad (6912)$$

$$\tau_{\alpha,i}^5 = \sum_{a \in V} {}^1T_{a,i} W_{a,\alpha}^4 \quad (2r_V N_o N_v) \quad (6925)$$

$$\tau_{\gamma,\alpha}^6 = \sum_{\beta \in B} X_{\alpha,\beta} \tau_{\gamma,\beta}^4 \tau_{\gamma,\beta}^5 \quad (3r_T r_V^2) \quad (6913)$$

$$\tau_{\alpha}^6 = \sum_{i \in O} W_{i,\alpha}^3 \tau_{\alpha,i}^5 \quad (2r_V N_o) \quad (6926)$$

$$\tau_{\gamma,\alpha}^7 = \sum_{\delta \in A} Z_{\delta,\gamma} \tau_{\delta,\alpha}^6 \quad (2r_T^2 r_V) \quad (6914)$$

$$\tau_{\alpha}^7 = \sum_{\beta \in B} \tau_{\beta}^6 X_{\alpha,\beta} \quad (2r_V^2) \quad (6927)$$



$$\tau^8_{i,a} = \sum_{\alpha \in B} \tau^7_{\alpha} W^1_{i,\alpha} W^2_{a,\alpha} \quad (3r_V N_o N_v) \quad (6928)$$

$$\tau^8_{\gamma,i} = \sum_{a \in V} Y^1_{a,\gamma} \tau^7_{i,a} \quad (2r_T N_o N_v) \quad (6941)$$

$$\tau^9_{\gamma,i} = \sum_{a \in V} Y^3_{a,\gamma} \tau^8_{i,a} \quad (2r_T N_o N_v) \quad (6929)$$

$$\tau^9_{\gamma,\delta,w} = \sum_{i \in O} \tau^8_{\gamma,i} \tau^3_{\delta,w,i} \quad (2r_D r_T^2 N_o) \quad (6942)$$

$$\tau^{10}_{\gamma,\delta,w} = \sum_{i \in O} \tau^9_{\gamma,i} \tau^4_{\delta,w,i} \quad (2r_D r_T^2 N_o) \quad (6930)$$

$$\tau^{10}_{\gamma,\delta,w} = \sum_{\epsilon \in A} Z_{\epsilon,\gamma} \tau^2_{\epsilon,\delta,w} \tau^9_{\epsilon,\delta,w} \quad (3r_D r_T^3) \quad (6943)$$

$${}^2R^z_{\gamma,\delta} \leftarrow - \sum_{\epsilon \in A} \sum_{w \in D} \tau^{10}_{\epsilon,\delta,w} \tau^2_{\epsilon,\gamma,w} \tau^3_{\epsilon,\delta,w} \quad (3r_D r_T^3) \quad (6931)$$

$${}^2R^z_{\gamma,\delta} \leftarrow - \sum_{\epsilon \in A} \sum_{w \in D} \tau^0_{\epsilon,\gamma,w} \tau^1_{\epsilon,\gamma,w} \tau^{10}_{\epsilon,\delta,w} \quad (3r_D r_T^3) \quad (6944)$$

Raw expression

$${}^2R^z_{\epsilon,\zeta} \leftarrow \sum_{i \in O} \sum_{j \in O} \sum_{k \in O} \sum_{l \in O} \sum_{a \in V} \sum_{b \in V} \sum_{c \in V} \sum_{d \in V} \frac{1}{2} \quad (6932)$$

$$\begin{aligned} & {}^1T_{a,k} {}^1T_{c,j} Y^{1,*}_{a,\epsilon} Y^{2,*}_{i,\epsilon} Y^{3,*}_{b,\zeta} \\ & Y^{4,*}_{j,\zeta} {}^2D^{a,i,b,j} {}^2T_{d,i,b,l} V_{k,d,l,c} \end{aligned}$$

Raw expression

$${}^2R^z_{\epsilon,\zeta} \leftarrow \sum_{i \in O} \sum_{j \in O} \sum_{k \in O} \sum_{l \in O} \sum_{a \in V} \sum_{b \in V} \sum_{c \in V} \sum_{d \in V} \frac{1}{2} \quad (6945)$$

$$\begin{aligned} & {}^1T_{a,k} {}^1T_{c,l} Y^{1,*}_{a,\epsilon} Y^{2,*}_{i,\epsilon} Y^{3,*}_{b,\zeta} \\ & Y^{4,*}_{j,\zeta} {}^2D^{a,i,b,j} {}^2T_{b,j,d,i} V_{k,c,l,d} \end{aligned}$$

Factorized expression

$$\tau^0_{\gamma,\delta,w} = \sum_{a \in V} {}^2D^1_{a,w} Y^3_{a,\gamma} Y^{1,*}_{a,\delta} \quad (3r_D r_T^2 N_v) \quad (6933)$$

$$\tau^0_{\gamma,\delta,w} = \sum_{a \in V} {}^2D^1_{a,w} Y^1_{a,\gamma} Y^{1,*}_{a,\delta} \quad (3r_D r_T^2 N_v) \quad (6946)$$

$$\tau^1_{\gamma,\delta,w} = \sum_{i \in O} {}^2D^2_{i,w} Y^4_{i,\gamma} Y^{2,*}_{i,\delta} \quad (3r_D r_T^2 N_o) \quad (6934)$$

$$\tau^1_{\alpha,i} = \sum_{a \in V} {}^1T_{a,i} W^2_{a,\alpha} \quad (2r_V N_o N_v) \quad (6947)$$

$$\tau^2_{\gamma,\delta,w} = \sum_{i \in O} {}^2D^4_{i,w} Y^2_{i,\gamma} Y^{4,*}_{i,\delta} \quad (3r_D r_T^2 N_o) \quad (6935)$$

$$\tau^2_{\alpha} = \sum_{i \in O} W^1_{i,\alpha} \tau^1_{\alpha,i} \quad (2r_V N_o) \quad (6948)$$

$$\tau^3_{\gamma,w,i} = \sum_{a \in V} {}^2D^3_{a,w} {}^1T_{a,i} Y^{3,*}_{a,\gamma} \quad (3r_D r_T N_o N_v) \quad (6936)$$

$$\tau^3_{\alpha} = \sum_{\beta \in B} \tau^2_{\beta} X_{\beta,\alpha} \quad (2r_V^2) \quad (6949)$$

$$\tau^4_{\alpha,i} = \sum_{a \in V} {}^1T_{a,i} W^4_{a,\alpha} \quad (2r_V N_o N_v) \quad (6937)$$

$$\tau^4_{i,a} = \sum_{\alpha \in B} \tau^3_{\alpha} W^3_{i,\alpha} W^4_{a,\alpha} \quad (3r_V N_o N_v) \quad (6950)$$

$$\tau^5_{\alpha} = \sum_{i \in O} W^3_{i,\alpha} \tau^4_{\alpha,i} \quad (2r_V N_o) \quad (6938)$$

$$\tau^5_{i,j} = \sum_{a \in V} {}^1T_{a,i} \tau^4_{j,a} \quad (2N_o^2 N_v) \quad (6951)$$

$$\tau^6_{\alpha} = \sum_{\beta \in B} \tau^5_{\beta} X_{\alpha,\beta} \quad (2r_V^2) \quad (6939)$$

$$\tau^6_{\gamma,i} = \sum_{j \in O} Y^2_{j,\gamma} \tau^5_{i,j} \quad (2r_T N_o^2) \quad (6952)$$

$$\tau^7_{i,a} = \sum_{\alpha \in B} \tau^6_{\alpha} W^1_{i,\alpha} W^2_{a,\alpha} \quad (3r_V N_o N_v) \quad (6940)$$

$$\tau^7_{\gamma,\delta,w} = \sum_{i \in O} {}^2D^2_{i,w} Y^{2,*}_{i,\delta} \tau^6_{\gamma,i} \quad (3r_D r_T^2 N_o) \quad (6953)$$

$$\tau_{\gamma,\delta,w}^8 = \sum_{\epsilon \in A} Z_{\epsilon,\gamma} \tau_{\epsilon,\delta,w}^0 \tau_{\epsilon,\delta,w}^7 \quad (3r_D r_T^3) \quad (6954)$$

$$\tau_{\gamma,\delta,w}^8 = \sum_{a \in V} {}^2D_{a,w}^3 Y_{a,\gamma}^1 Y_{a,\delta}^{3,*} \quad (3r_D r_T^2 N_v) \quad (6967)$$

$$\tau_{\gamma,\delta,w}^9 = \sum_{a \in V} {}^2D_{a,w}^3 Y_{a,\gamma}^3 Y_{a,\delta}^{3,*} \quad (3r_D r_T^2 N_v) \quad (6955)$$

$$\tau_{\gamma,\delta,w}^9 = \sum_{i \in O} {}^2D_{i,w}^4 Y_{i,\gamma}^2 Y_{i,\delta}^{4,*} \quad (3r_D r_T^2 N_o) \quad (6968)$$

$$\tau_{\gamma,\delta,w}^{10} = \sum_{i \in O} {}^2D_{i,w}^4 Y_{i,\gamma}^4 Y_{i,\delta}^{4,*} \quad (3r_D r_T^2 N_o) \quad (6956)$$

$$\tau_{\gamma,\delta,w}^{10} = \sum_{\epsilon \in A} Z_{\epsilon,\gamma} \tau_{\epsilon,\delta,w}^8 \tau_{\epsilon,\delta,w}^9 \quad (3r_D r_T^3) \quad (6969)$$

$${}^2R_{\gamma,\delta}^z \leftarrow - \sum_{\epsilon \in A} \sum_{w \in D} \tau_{\epsilon,\delta,w}^{10} \tau_{\epsilon,\gamma,w}^8 \tau_{\epsilon,\delta,w}^9 \quad (3r_D r_T^3) \quad (6957)$$

$${}^2R_{\gamma,\delta}^z \leftarrow - \sum_{\epsilon \in A} \sum_{w \in D} \tau_{\epsilon,\gamma,w}^0 \tau_{\epsilon,\delta,w}^{10} \tau_{\epsilon,\gamma,w}^7 \quad (3r_D r_T^3) \quad (6970)$$

Raw expression

$${}^2R_{\epsilon,\zeta}^z \leftarrow \sum_{i \in O} \sum_{j \in O} \sum_{k \in O} \sum_{l \in O} \sum_{a \in V} \sum_{b \in V} \sum_{c \in V} \sum_{d \in V} \frac{1}{2} \quad (6958)$$

$$\begin{aligned} & {}^1T_{a,k} \quad {}^1T_{c,l} \quad Y_{a,\epsilon}^{1,*} \quad Y_{i,\epsilon}^{2,*} \quad Y_{b,\zeta}^{3,*} \\ & Y_{j,\zeta}^{4,*} \quad {}^2D_{a,i,b,j} \quad {}^2T_{d,i,b,j} \quad V_{k,c,l,d} \end{aligned}$$

Raw expression

$${}^2R_{\epsilon,\zeta}^z \leftarrow \sum_{i \in O} \sum_{j \in O} \sum_{k \in O} \sum_{l \in O} \sum_{a \in V} \sum_{b \in V} \sum_{c \in V} \sum_{d \in V} \frac{1}{2} \quad (6971)$$

$$\begin{aligned} & {}^1T_{b,k} \quad {}^1T_{c,i} \quad Y_{a,\epsilon}^{1,*} \quad Y_{i,\epsilon}^{2,*} \quad Y_{b,\zeta}^{3,*} \\ & Y_{j,\zeta}^{4,*} \quad {}^2D_{a,i,b,j} \quad {}^2T_{a,l,d,j} \quad V_{k,d,l,c} \end{aligned}$$

Factorized expression

$$\tau_{\gamma,\delta,w}^0 = \sum_{a \in V} {}^2D_{a,w}^1 Y_{a,\gamma}^3 Y_{a,\delta}^{1,*} \quad (3r_D r_T^2 N_v) \quad (6959)$$

$$\tau_{\gamma,\delta,w}^0 = \sum_{a \in V} {}^2D_{a,w}^1 Y_{a,\gamma}^1 Y_{a,\delta}^{1,*} \quad (3r_D r_T^2 N_v) \quad (6972)$$

$$\tau_{\alpha,i}^1 = \sum_{a \in V} {}^1T_{a,i} W_{a,\alpha}^2 \quad (2r_V N_o N_v) \quad (6960)$$

$$\tau_{\gamma,\delta,w}^1 = \sum_{i \in O} {}^2D_{i,w}^2 Y_{i,\gamma}^2 Y_{i,\delta}^{2,*} \quad (3r_D r_T^2 N_o) \quad (6973)$$

$$\tau_{\alpha}^2 = \sum_{i \in O} W_{i,\alpha}^1 \tau_{\alpha,i}^1 \quad (2r_V N_o) \quad (6961)$$

$$\tau_{\gamma,\delta,w}^2 = \sum_{\epsilon \in A} Z_{\epsilon,\gamma} \tau_{\epsilon,\delta,w}^0 \tau_{\epsilon,\delta,w}^1 \quad (3r_D r_T^3) \quad (6974)$$

$$\tau_{\alpha}^3 = \sum_{\beta \in B} \tau_{\beta}^2 X_{\beta,\alpha} \quad (2r_V^2) \quad (6962)$$

$$\tau_{\gamma,\delta,w}^3 = \sum_{a \in V} {}^2D_{a,w}^3 Y_{a,\gamma}^3 Y_{a,\delta}^{3,*} \quad (3r_D r_T^2 N_v) \quad (6975)$$

$$\tau_{i,a}^4 = \sum_{\alpha \in B} \tau_{\alpha}^3 W_{i,\alpha}^3 W_{a,\alpha}^4 \quad (3r_V N_o N_v) \quad (6963)$$

$$\tau_{\alpha,i}^4 = \sum_{a \in V} {}^1T_{a,i} W_{a,\alpha}^2 \quad (2r_V N_o N_v) \quad (6976)$$

$$\tau_{i,j}^5 = \sum_{a \in V} {}^1T_{a,i} \tau_{j,a}^4 \quad (2N_o^2 N_v) \quad (6964)$$

$$\tau_{\alpha}^5 = \sum_{i \in O} W_{i,\alpha}^1 \tau_{\alpha,i}^4 \quad (2r_V N_o) \quad (6977)$$

$$\tau_{\gamma,i}^6 = \sum_{j \in O} Y_{j,\gamma}^4 \tau_{i,j}^5 \quad (2r_T N_o^2) \quad (6965)$$

$$\tau_{\alpha}^6 = \sum_{\beta \in B} \tau_{\beta}^5 X_{\beta,\alpha} \quad (2r_V^2) \quad (6978)$$

$$\tau_{\gamma,\delta,w}^7 = \sum_{i \in O} {}^2D_{i,w}^2 Y_{i,\gamma}^{2,*} \tau_{\gamma,i}^6 \quad (3r_D r_T^2 N_o) \quad (6966)$$

$$\tau_{i,a}^7 = \sum_{\alpha \in B} \tau_{\alpha}^6 W_{i,\alpha}^3 W_{a,\alpha}^4 \quad (3r_V N_o N_v) \quad (6979)$$

$$\tau^8_{i,j} = \sum_{a \in V} {}^1T_{a,i} \tau^7_{j,a} \quad (2N_o^2 N_v) \quad (6980)$$

$$\tau^8_{\gamma,i} = \sum_{j \in O} Y^2_{j,\gamma} \tau^7_{i,j} \quad (2r_T N_o^2) \quad (6993)$$

$$\tau^9_{\gamma,i} = \sum_{j \in O} Y^4_{j,\gamma} \tau^8_{i,j} \quad (2r_T N_o^2) \quad (6981)$$

$$\tau^9_{\gamma,\delta,w} = \sum_{i \in O} {}^2D^4_{i,w} Y^{4,*}_{i,\delta} \tau^8_{\gamma,i} \quad (3r_D r_T^2 N_o) \quad (6994)$$

$$\tau^{10}_{\gamma,\delta,w} = \sum_{i \in O} {}^2D^4_{i,w} Y^{4,*}_{i,\delta} \tau^9_{\gamma,i} \quad (3r_D r_T^2 N_o) \quad (6982)$$

$$\tau^{10}_{\gamma,\delta,w} = \sum_{\epsilon \in A} Z_{\epsilon,\gamma} \tau^2_{\epsilon,\delta,w} \tau^9_{\epsilon,\delta,w} \quad (3r_D r_T^3) \quad (6995)$$

$${}^2R^z_{\gamma,\delta} \leftarrow - \sum_{\epsilon \in A} \sum_{w \in D} \tau^{10}_{\epsilon,\delta,w} \tau^2_{\epsilon,\gamma,w} \tau^3_{\epsilon,\delta,w} \quad (3r_D r_T^3) \quad (6983)$$

$${}^2R^z_{\gamma,\delta} \leftarrow - \sum_{\epsilon \in A} \sum_{w \in D} \tau^0_{\epsilon,\gamma,w} \tau^1_{\epsilon,\gamma,w} \tau^{10}_{\epsilon,\delta,w} \quad (3r_D r_T^3) \quad (6996)$$

Raw expression

$${}^2R^z_{\epsilon,\zeta} \leftarrow \sum_{i \in O} \sum_{j \in O} \sum_{k \in O} \sum_{l \in O} \sum_{a \in V} \sum_{b \in V} \sum_{c \in V} \sum_{d \in V} \frac{1}{2} \quad (6984)$$

$${}^1T_{b,k} \quad {}^1T_{c,i} \quad Y^{1,*}_{a,\epsilon} \quad Y^{2,*}_{i,\epsilon} \quad Y^{3,*}_{b,\zeta} \quad Y^{4,*}_{j,\zeta} \quad {}^2D^{a,i,b,j} \quad {}^2T_{d,j,a,l} \quad V_{k,d,l,c}$$

Raw expression

$${}^2R^z_{\epsilon,\zeta} \leftarrow \sum_{i \in O} \sum_{j \in O} \sum_{k \in O} \sum_{l \in O} \sum_{a \in V} \sum_{b \in V} \sum_{c \in V} \sum_{d \in V} \frac{1}{2} \quad (6997)$$

$${}^1T_{b,k} \quad {}^1T_{c,j} \quad Y^{1,*}_{a,\epsilon} \quad Y^{2,*}_{i,\epsilon} \quad Y^{3,*}_{b,\zeta} \quad Y^{4,*}_{j,\zeta} \quad {}^2D^{a,i,b,j} \quad {}^2T_{a,i,d,l} \quad V_{k,d,l,c}$$

Factorized expression

$$\tau^0_{\gamma,\delta,w} = \sum_{a \in V} {}^2D^1_{a,w} Y^3_{a,\gamma} Y^{1,*}_{a,\delta} \quad (3r_D r_T^2 N_v) \quad (6985)$$

$$\tau^0_{\gamma,w,i} = \sum_{a \in V} {}^2D^3_{a,w} {}^1T_{a,i} Y^{3,*}_{a,\gamma} \quad (3r_D r_T N_o N_v) \quad (6998)$$

$$\tau^1_{\gamma,\delta,w} = \sum_{i \in O} {}^2D^2_{i,w} Y^4_{i,\gamma} Y^{2,*}_{i,\delta} \quad (3r_D r_T^2 N_o) \quad (6986)$$

$$\tau^1_{\gamma,w,i} = \sum_{a \in V} {}^2D^1_{a,w} {}^1T_{a,i} Y^{1,*}_{a,\gamma} \quad (3r_D r_T N_o N_v) \quad (6999)$$

$$\tau^2_{\gamma,\delta,w} = \sum_{a \in V} {}^2D^3_{a,w} Y^1_{a,\gamma} Y^{3,*}_{a,\delta} \quad (3r_D r_T^2 N_v) \quad (6987)$$

$$\tau^3_{\alpha,i} = \sum_{a \in V} {}^1T_{a,i} W^2_{a,\alpha} \quad (2r_V N_o N_v) \quad (6988)$$

$$\tau^2_{\gamma,\alpha} = \sum_{a \in V} W^2_{a,\alpha} Y^1_{a,\gamma} \quad (2r_T r_V N_v) \quad (7000)$$

$$\tau^4_{\alpha} = \sum_{i \in O} W^1_{i,\alpha} \tau^3_{\alpha,i} \quad (2r_V N_o) \quad (6989)$$

$$\tau^3_{\gamma,\alpha,i} = \sum_{\beta \in B} W^1_{i,\beta} X_{\beta,\alpha} \tau^2_{\gamma,\beta} \quad (3r_T r_V^2 N_o) \quad (7001)$$

$$\tau^5_{\alpha} = \sum_{\beta \in B} \tau^4_{\beta} X_{\beta,\alpha} \quad (2r_V^2) \quad (6990)$$

$$\tau^4_{\gamma,\alpha} = \sum_{a \in V} W^4_{a,\alpha} Y^3_{a,\gamma} \quad (2r_T r_V N_v) \quad (7002)$$

$$\tau^6_{i,a} = \sum_{\alpha \in B} \tau^5_{\alpha} W^3_{i,\alpha} W^4_{a,\alpha} \quad (3r_V N_o N_v) \quad (6991)$$

$$\tau^5_{\gamma,\alpha,i} = \sum_{\delta \in A} Z_{\gamma,\delta} Y^4_{i,\delta} \tau^4_{\delta,\alpha} \quad (3r_T^2 r_V N_o) \quad (7003)$$

$$\tau^7_{i,j} = \sum_{a \in V} {}^1T_{a,i} \tau^6_{j,a} \quad (2N_o^2 N_v) \quad (6992)$$

$$\tau^6_{\gamma,i,j,k} = \sum_{\alpha \in B} W^3_{j,\alpha} \tau^3_{\gamma,\alpha,i} \tau^5_{\gamma,\alpha,k} \quad (3r_T r_V N_o^3) \quad (7004)$$

$$\tau^7_{i,j,k,l} = \sum_{\gamma \in A} Y^2_{k,\gamma} \tau^6_{\gamma,i,j,l} \quad (2r_T N_o^4) \quad (7005) \quad \tau^8_{\gamma,w,i,j} = \sum_{k \in O} \sum_{l \in O} {}^2D^2_{k,w} Y^{2,*}_{k,\gamma} \tau^1_{\gamma,w,l} \tau^7_{l,i,j,k} \quad (4r_D r_T N_o^4) \quad (7017)$$

$$\tau^8_{\gamma,w,i,j} = \sum_{k \in O} \sum_{l \in O} {}^2D^2_{k,w} Y^{2,*}_{k,\gamma} \tau^1_{\gamma,w,l} \tau^7_{l,i,k,j} \quad (4r_D r_T N_o^4) \quad (7006) \quad {}^2R^z_{\gamma,\delta} \leftarrow \sum_{w \in D} \sum_{i \in O} \sum_{j \in O} \frac{1}{2} {}^2D^4_{i,w} Y^{4,*}_{i,\delta} \tau^0_{\delta,w,j} \tau^8_{\gamma,w,j,i} \quad (4r_D r_T^2 N_o^2) \quad (7018)$$

$${}^2R^z_{\gamma,\delta} \leftarrow \sum_{w \in D} \sum_{i \in O} \sum_{j \in O} \frac{1}{2} {}^2D^4_{i,w} Y^{4,*}_{i,\delta} \tau^0_{\delta,w,j} \tau^8_{\gamma,w,j,i} \quad (4r_D r_T^2 N_o^2) \quad \text{Raw expression} \quad (7007)$$

Raw expression

$${}^2R^z_{\epsilon,\zeta} \leftarrow \sum_{i \in O} \sum_{j \in O} \sum_{k \in O} \sum_{l \in O} \sum_{a \in V} \sum_{b \in V} \sum_{c \in V} \sum_{d \in V} \frac{1}{2} \quad (7008) \quad {}^2R^z_{\epsilon,\zeta} \leftarrow \sum_{i \in O} \sum_{j \in O} \sum_{k \in O} \sum_{l \in O} \sum_{a \in V} \sum_{b \in V} \sum_{c \in V} \sum_{d \in V} \frac{1}{2} \quad (7019)$$

$$\begin{aligned} & {}^1T_{b,k} \quad {}^1T_{c,j} \quad Y^{1,*}_{a,\epsilon} \quad Y^{2,*}_{i,\epsilon} \quad Y^{3,*}_{b,\zeta} \\ & Y^{4,*}_{j,\zeta} \quad {}^2D^{a,i,b,j} \quad {}^2T_{a,l,d,i} \quad V_{k,c,l,d} \end{aligned}$$

Factorized expression

Factorized expression

$$\tau^0_{\gamma,\delta,w} = \sum_{a \in V} {}^2D^3_{a,w} Y^1_{a,\gamma} Y^{3,*}_{a,\delta} \quad (3r_D r_T^2 N_v) \quad (7020)$$

$$\tau^0_{\gamma,w,i} = \sum_{a \in V} {}^2D^3_{a,w} {}^1T_{a,i} Y^{3,*}_{a,\gamma} \quad (3r_D r_T N_o N_v) \quad (7009)$$

$$\tau^1_{\gamma,\alpha} = \sum_{i \in O} W^3_{i,\alpha} Y^2_{i,\gamma} \quad (2r_T r_V N_o) \quad (7021)$$

$$\tau^1_{\gamma,w,i} = \sum_{a \in V} {}^2D^1_{a,w} {}^1T_{a,i} Y^{1,*}_{a,\gamma} \quad (3r_D r_T N_o N_v) \quad (7010)$$

$$\tau^2_{\gamma,\alpha} = \sum_{a \in V} W^4_{a,\alpha} Y^3_{a,\gamma} \quad (2r_T r_V N_v) \quad (7022)$$

$$\tau^2_{\gamma,\alpha} = \sum_{a \in V} W^4_{a,\alpha} Y^1_{a,\gamma} \quad (2r_T r_V N_v) \quad (7011)$$

$$\tau^3_{\gamma,\alpha,i} = \sum_{\delta \in A} Z_{\gamma,\delta} Y^4_{i,\delta} \tau^2_{\delta,\alpha} \quad (3r_T^2 r_V N_o) \quad (7023)$$

$$\tau^3_{\gamma,\alpha,i} = \sum_{\beta \in B} X_{\alpha,\beta} W^3_{i,\beta} \tau^2_{\gamma,\beta} \quad (3r_T r_V^2 N_o) \quad (7012)$$

$$\tau^4_{\gamma,\alpha,w} = \sum_{\delta \in A} \sum_{i \in O} {}^2D^4_{i,w} Y^{4,*}_{i,\gamma} \tau^1_{\delta,\alpha} \tau^0_{\delta,\gamma,w} \tau^3_{\delta,\alpha,i} \quad (5r_D r_T^2 r_V N_o) \quad (7024)$$

$$\tau^4_{\gamma,\alpha} = \sum_{a \in V} W^2_{a,\alpha} Y^3_{a,\gamma} \quad (2r_T r_V N_v) \quad (7013)$$

$$\tau^5_{\gamma,\alpha,w} = \sum_{\beta \in B} X_{\alpha,\beta} \tau^4_{\gamma,\beta,w} \quad (2r_D r_T r_V^2) \quad (7025)$$

$$\tau^5_{\gamma,\alpha,i} = \sum_{\delta \in A} Z_{\gamma,\delta} Y^4_{i,\delta} \tau^4_{\delta,\alpha} \quad (3r_T^2 r_V N_o) \quad (7014)$$

$$\tau^6_{\alpha,i} = \sum_{a \in V} {}^1T_{a,i} W^2_{a,\alpha} \quad (2r_V N_o N_v) \quad (7026)$$

$$\tau^6_{\gamma,i,j,k} = \sum_{\alpha \in B} W^1_{i,\alpha} \tau^3_{\gamma,\alpha,j} \tau^5_{\gamma,\alpha,k} \quad (3r_T r_V N_o^3) \quad (7015)$$

$$\tau^7_{\gamma,\alpha,w} = \sum_{i \in O} {}^2D^2_{i,w} Y^{2,*}_{i,\gamma} \tau^6_{\alpha,i} \quad (3r_D r_T r_V N_o) \quad (7027)$$

$$\tau^7_{i,j,k,l} = \sum_{\gamma \in A} Y^2_{k,\gamma} \tau^6_{\gamma,i,j,l} \quad (2r_T N_o^4) \quad (7016)$$

$$\tau^8_{\gamma,w,i} = \sum_{a \in V} {}^2D^1_{a,w} {}^1T_{a,i} Y^{1,*}_{a,\gamma} \quad (3r_D r_T N_o N_v) \quad (7028)$$

$$\tau_{\gamma,\alpha,w}^9 = \sum_{i \in O} W_{i,\alpha}^1 \tau_{\gamma,w,i}^8 \quad (2r_D r_T r_V N_o) \quad (7029)$$

$${}^2R_{\gamma,\delta}^z \leftarrow \sum_{\alpha \in B} \sum_{w \in D} \frac{1}{2} \tau_{\delta,\alpha,w}^5 \tau_{\gamma,\alpha,w}^7 \tau_{\gamma,\alpha,w}^9 \quad (3r_D r_T^2 r_V) \quad (7042)$$

$${}^2R_{\gamma,\delta}^z \leftarrow \sum_{\alpha \in B} \sum_{w \in D} \frac{1}{2} \tau_{\delta,\alpha,w}^5 \tau_{\gamma,\alpha,w}^7 \tau_{\gamma,\alpha,w}^9 \quad (3r_D r_T^2 r_V) \quad (7030)$$

Raw expression

$${}^2R_{\epsilon,\zeta}^z \leftarrow \sum_{i \in O} \sum_{j \in O} \sum_{k \in O} \sum_{l \in O} \sum_{a \in V} \sum_{b \in V} \sum_{c \in V} \sum_{d \in V} \frac{1}{2} \quad (7031)$$

$${}^1T_{b,k} {}^1T_{c,j} Y_{a,\epsilon}^{1,*} Y_{i,\epsilon}^{2,*} Y_{b,\zeta}^{3,*} Y_{j,\zeta}^{4,*} {}^2D^{a,i,b,j} {}^2T_{d,l,a,i} V_{k,d,l,c}$$

Factorized expression

$$\tau_{\gamma,\delta,w}^0 = \sum_{a \in V} {}^2D_{a,w}^3 Y_{a,\gamma}^3 Y_{a,\delta}^{3,*} \quad (3r_D r_T^2 N_v) \quad (7032)$$

$$\tau_{\gamma,\alpha}^1 = \sum_{a \in V} W_{a,\alpha}^4 Y_{a,\gamma}^1 \quad (2r_T r_V N_v) \quad (7033)$$

$$\tau_{\gamma,\alpha,i}^2 = \sum_{\delta \in A} Y_{i,\delta}^2 Z_{\delta,\gamma} \tau_{\delta,\alpha}^1 \quad (3r_T^2 r_V N_o) \quad (7034)$$

$$\tau_{\gamma,\alpha}^3 = \sum_{i \in O} W_{i,\alpha}^3 Y_{i,\gamma}^4 \quad (2r_T r_V N_o) \quad (7035)$$

$$\tau_{\gamma,\alpha,w}^4 = \sum_{\delta \in A} \sum_{i \in O} {}^2D_{i,w}^4 Y_{i,\gamma}^{4,*} \tau_{i,\gamma}^3 \tau_{\delta,\alpha}^0 \tau_{\delta,\gamma,w}^0 \tau_{\delta,\alpha,i}^2 \quad (5r_D r_T^2 r_V N_o) \tau_{\alpha,i}^4 = \sum_{a \in V} {}^1T_{a,i} W_{a,\alpha}^4 \quad (2r_V N_o N_v) \quad (7048)$$

$$\tau_{\gamma,\alpha,w}^5 = \sum_{\beta \in B} X_{\alpha,\beta} \tau_{\gamma,\beta,w}^4 \quad (2r_D r_T r_V^2) \quad (7037)$$

$$\tau_{\alpha,i}^6 = \sum_{a \in V} {}^1T_{a,i} W_{a,\alpha}^2 \quad (2r_V N_o N_v) \quad (7038)$$

$$\tau_{\gamma,\alpha,w}^7 = \sum_{i \in O} {}^2D_{i,w}^2 Y_{i,\gamma}^{2,*} \tau_{i,\gamma}^6 \tau_{\alpha,i}^6 \quad (3r_D r_T r_V N_o) \quad (7039)$$

$$\tau_{\gamma,w,i}^8 = \sum_{a \in V} {}^2D_{a,w}^1 T_{a,i} Y_{a,\gamma}^{1,*} \quad (3r_D r_T N_o N_v) \quad (7040)$$

$$\tau_{\gamma,\alpha,w}^9 = \sum_{i \in O} W_{i,\alpha}^1 \tau_{\gamma,w,i}^8 \quad (2r_D r_T r_V N_o) \quad (7041)$$

Raw expression

$${}^2R_{\epsilon,\zeta}^z \leftarrow \sum_{i \in O} \sum_{j \in O} \sum_{k \in O} \sum_{l \in O} \sum_{a \in V} \sum_{b \in V} \sum_{c \in V} \sum_{d \in V} \frac{1}{2} \quad (7043)$$

$${}^1T_{b,k} {}^1T_{c,l} Y_{a,\epsilon}^{1,*} Y_{i,\epsilon}^{2,*} Y_{b,\zeta}^{3,*} Y_{j,\zeta}^{4,*} {}^2D^{a,i,b,j} {}^2T_{a,i,d,j} V_{k,c,l,d}$$

Factorized expression

$$\tau_{\gamma,\delta,w}^0 = \sum_{a \in V} {}^2D_{a,w}^3 Y_{a,\gamma}^1 Y_{a,\delta}^{3,*} \quad (3r_D r_T^2 N_v) \quad (7044)$$

$$\tau_{\gamma,\delta,w}^1 = \sum_{i \in O} {}^2D_{i,w}^4 Y_{i,\gamma}^2 Y_{i,\delta}^{4,*} \quad (3r_D r_T^2 N_o) \quad (7045)$$

$$\tau_{\gamma,w,i}^2 = \sum_{a \in V} {}^2D_{a,w}^1 T_{a,i} Y_{a,\gamma}^{1,*} \quad (3r_D r_T N_o N_v) \quad (7046)$$

$$\tau_{\gamma,\alpha}^3 = \sum_{a \in V} W_{a,\alpha}^2 Y_{a,\gamma}^3 \quad (2r_T r_V N_v) \quad (7047)$$

$$\tau_{\alpha,i,j}^5 = \sum_{\beta \in B} X_{\alpha,\beta} W_{j,\beta}^3 \tau_{\beta,i}^4 \quad (3r_V^2 N_o^2) \quad (7049)$$

$$\tau_{\gamma,\alpha,i}^6 = \sum_{j \in O} Y_{j,\gamma}^4 \tau_{\alpha,i,j}^5 \quad (2r_T r_V N_o^2) \quad (7050)$$

$$\tau_{\gamma,i,j}^7 = \sum_{\alpha \in B} W_{j,\alpha}^1 \tau_{\gamma,\alpha}^3 \tau_{\gamma,\alpha,i}^6 \quad (3r_T r_V N_o^2) \quad (7051)$$

$$\tau_{\gamma,i,j}^8 = \sum_{\delta \in A} Z_{\gamma,\delta} \tau_{\delta,i,j}^7 \quad (2r_T^2 N_o^2) \quad (7052)$$

$$\tau_{\gamma,\delta,w}^9 = \sum_{i \in O} \sum_{j \in O} {}^2D_{i,w}^2 Y_{i,\delta}^{2,*} \tau_{\delta,w,j}^2 \tau_{\gamma,i,j}^8 \quad (4r_D r_T^2 N_o^2) \quad (7053)$$

$${}^2R^z_{\gamma,\delta} \leftarrow \sum_{\epsilon \in A} \sum_{w \in D} \frac{1}{2} \tau^0_{\epsilon,\delta,w} \tau^1_{\epsilon,\delta,w} \tau^9_{\epsilon,\gamma,w} \quad (3r_D r_T^3) \quad (7054)$$

Raw expression

$${}^2R^z_{\epsilon,\zeta} \leftarrow \sum_{i \in O} \sum_{j \in O} \sum_{k \in O} \sum_{l \in O} \sum_{a \in V} \sum_{b \in V} \sum_{c \in V} \sum_{d \in V} \frac{1}{2} \quad (7055)$$

$${}^1T_{b,k} \quad {}^1T_{c,l} \quad Y^{1,*}_{a,\epsilon} \quad Y^{2,*}_{i,\epsilon} \quad Y^{3,*}_{b,\zeta}$$

$$Y^{4,*}_{j,\zeta} \quad {}^2D^{a,i,b,j} \quad {}^2T_{d,j,a,i} \quad V_{k,c,l,d}$$

Factorized expression

$$\tau^0_{\gamma,\delta,w} = \sum_{a \in V} {}^2D^3_{a,w} Y^3_{a,\gamma} Y^{3,*}_{a,\delta} \quad (3r_D r_T^2 N_v) \quad (7056)$$

$$\tau^1_{\gamma,\delta,w} = \sum_{i \in O} {}^2D^4_{i,w} Y^4_{i,\gamma} Y^{4,*}_{i,\delta} \quad (3r_D r_T^2 N_o) \quad (7057)$$

$$\tau^2_{\gamma,w,i} = \sum_{a \in V} {}^2D^1_{a,w} {}^1T_{a,i} Y^{1,*}_{a,\gamma} \quad (3r_D r_T N_o N_v) \quad (7058)$$

$$\tau^3_{\gamma,\alpha} = \sum_{a \in V} W^2_{a,\alpha} Y^1_{a,\gamma} \quad (2r_T r_V N_v) \quad (7059)$$

$$\tau^4_{\alpha,i} = \sum_{a \in V} {}^1T_{a,i} W^4_{a,\alpha} \quad (2r_V N_o N_v) \quad (7060)$$

$$\tau^5_{\alpha,i,j} = \sum_{\beta \in B} X_{\alpha,\beta} W^3_{j,\beta} \tau^4_{\beta,i} \quad (3r_V^2 N_o^2) \quad (7061)$$

$$\tau^6_{\gamma,\alpha,i} = \sum_{j \in O} Y^2_{j,\gamma} \tau^5_{\alpha,i,j} \quad (2r_T r_V N_o^2) \quad (7062)$$

$$\tau^7_{\gamma,i,j} = \sum_{\alpha \in B} W^1_{j,\alpha} \tau^3_{\gamma,\alpha} \tau^6_{\gamma,\alpha,i} \quad (3r_T r_V N_o^2) \quad (7063)$$

$$\tau^8_{\gamma,i,j} = \sum_{\delta \in A} Z_{\delta,\gamma} \tau^7_{\delta,i,j} \quad (2r_T^2 N_o^2) \quad (7064)$$

$$\tau^9_{\gamma,\delta,w} = \sum_{i \in O} \sum_{j \in O} {}^2D^2_{i,w} Y^{2,*}_{i,\delta} \tau^2_{\delta,w,j} \tau^8_{\gamma,i,j} \quad (4r_D r_T^2 N_o^2) \quad (7065)$$

$${}^2R^z_{\gamma,\delta} \leftarrow \sum_{\epsilon \in A} \sum_{w \in D} \frac{1}{2} \tau^0_{\epsilon,\delta,w} \tau^1_{\epsilon,\delta,w} \tau^9_{\epsilon,\gamma,w} \quad (3r_D r_T^3) \quad (7066)$$

Raw expression

$${}^2R^z_{\epsilon,\zeta} \leftarrow \sum_{i \in O} \sum_{j \in O} \sum_{k \in O} \sum_{l \in O} \sum_{a \in V} \sum_{b \in V} \sum_{c \in V} \sum_{d \in V} \frac{1}{2} \quad (7067)$$

$${}^1T_{c,i} \quad {}^1T_{d,j} \quad Y^{1,*}_{a,\epsilon} \quad Y^{2,*}_{i,\epsilon} \quad Y^{3,*}_{b,\zeta}$$

$$Y^{4,*}_{j,\zeta} \quad {}^2D^{a,i,b,j} \quad {}^2T_{a,k,b,l} \quad V_{k,c,l,d}$$

Factorized expression

$$\tau^0_{\gamma,w,i} = \sum_{a \in V} {}^2D^1_{a,w} {}^1T_{a,i} Y^{1,*}_{a,\gamma} \quad (3r_D r_T N_o N_v) \quad (7068)$$

$$\tau^1_{\gamma,\alpha} = \sum_{a \in V} W^2_{a,\alpha} Y^3_{a,\gamma} \quad (2r_T r_V N_v) \quad (7069)$$

$$\tau^2_{\gamma,\alpha,i} = \sum_{\delta \in A} Z_{\gamma,\delta} Y^4_{i,\delta} \tau^1_{\delta,\alpha} \quad (3r_T^2 r_V N_o) \quad (7070)$$

$$\tau^3_{\gamma,\delta,w} = \sum_{a \in V} {}^2D^3_{a,w} Y^1_{a,\gamma} Y^{3,*}_{a,\delta} \quad (3r_D r_T^2 N_v) \quad (7071)$$

$$\tau^4_{\alpha,i} = \sum_{a \in V} {}^1T_{a,i} W^4_{a,\alpha} \quad (2r_V N_o N_v) \quad (7072)$$

$$\tau^5_{\alpha,i,j} = \sum_{\beta \in B} X_{\alpha,\beta} W^3_{j,\beta} \tau^4_{\beta,i} \quad (3r_V^2 N_o^2) \quad (7073)$$

$$\tau^6_{\gamma,\alpha,i} = \sum_{j \in O} Y^2_{j,\gamma} \tau^5_{\alpha,i,j} \quad (2r_T r_V N_o^2) \quad (7074)$$

$$\tau^7_{\gamma,\delta,\alpha,w} = \sum_{i \in O} {}^2D^4_{i,w} Y^{4,*}_{i,\delta} \tau^3_{\gamma,\delta,w} \tau^6_{\gamma,\alpha,i} \quad (4r_D r_T^2 r_V N_o) \quad (7075)$$

$$\tau^8_{\gamma,\alpha,w,i} = \sum_{\delta \in A} \tau^2_{\delta,\alpha,i} \tau^7_{\delta,\gamma,\alpha,w} \quad (2r_D r_T^2 r_V N_o) \quad (7076)$$

$$\tau^9_{\gamma,w,i,j} = \sum_{\alpha \in B} W^1_{i,\alpha} \tau^8_{\gamma,\alpha,w,j} \quad (2r_D r_T r_V N_o^2) \quad (7077)$$

$${}^2R^z_{\gamma,\delta} \leftarrow \sum_{w \in D} \sum_{i \in O} \sum_{j \in O} \frac{1}{2} {}^2D^2_{i,w} Y^{2,*}_{i,\gamma} \tau^0_{\gamma,w,j} \tau^9_{\delta,w,j,i} \quad (4r_D r_T^2 N_o^2) \quad (7078)$$

Raw expression

$${}^2R^z_{\epsilon,\zeta} \leftarrow \sum_{i \in O} \sum_{j \in O} \sum_{k \in O} \sum_{l \in O} \sum_{a \in V} \sum_{b \in V} \sum_{c \in V} \sum_{d \in V} \frac{1}{2} \quad (7079)$$

$$\begin{aligned} & {}^1T_{c,i} \quad {}^1T_{d,k} \quad Y^{1,*}_{a,\epsilon} \quad Y^{2,*}_{i,\epsilon} \quad Y^{3,*}_{b,\zeta} \\ & Y^{4,*}_{j,\zeta} \quad {}^2D^{a,i,b,j} \quad {}^2T_{a,l,b,j} \quad V_{k,c,l,d} \end{aligned}$$

Factorized expression

$$\tau^0_{\gamma,w,i} = \sum_{a \in V} {}^2D^1_{a,w} {}^1T_{a,i} Y^{1,*}_{a,\gamma} \quad (3r_D r_T N_o N_v) \quad (7080)$$

$$\tau^1_{\gamma,\alpha} = \sum_{a \in V} W^2_{a,\alpha} Y^1_{a,\gamma} \quad (2r_T r_V N_v) \quad (7081)$$

$$\tau^2_{\gamma,\alpha,i} = \sum_{\delta \in A} Y^2_{i,\delta} Z_{\delta,\gamma} \tau^1_{\delta,\alpha} \quad (3r_T^2 r_V N_o) \quad (7082)$$

$$\tau^3_{\gamma,\delta,w} = \sum_{a \in V} {}^2D^3_{a,w} Y^3_{a,\gamma} Y^{3,*}_{a,\delta} \quad (3r_D r_T^2 N_v) \quad (7083)$$

$$\tau^4_{\alpha,i} = \sum_{a \in V} {}^1T_{a,i} W^4_{a,\alpha} \quad (2r_V N_o N_v) \quad (7084)$$

$$\tau^5_{\alpha,i,j} = \sum_{\beta \in B} X_{\alpha,\beta} W^3_{j,\beta} \tau^4_{\beta,i} \quad (3r_V^2 N_o^2) \quad (7085)$$

$$\tau^6_{\gamma,\alpha,i} = \sum_{j \in O} Y^4_{j,\gamma} \tau^5_{\alpha,i,j} \quad (2r_T r_V N_o^2) \quad (7086)$$

$$\tau^7_{\gamma,\delta,\alpha,w} = \sum_{i \in O} {}^2D^4_{i,w} Y^{4,*}_{i,\delta} \tau^3_{\gamma,\delta,w} \tau^6_{\gamma,\alpha,i} \quad (4r_D r_T^2 r_V N_o) \quad (7087)$$

$$\tau^8_{\gamma,\alpha,w,i} = \sum_{\delta \in A} \tau^2_{\delta,\alpha,i} \tau^7_{\delta,\gamma,\alpha,w} \quad (2r_D r_T^2 r_V N_o) \quad (7088)$$

$$\tau^9_{\gamma,w,i,j} = \sum_{\alpha \in B} W^1_{i,\alpha} \tau^8_{\gamma,\alpha,w,j} \quad (2r_D r_T r_V N_o^2) \quad (7089)$$

Raw expression

$${}^2R^z_{\epsilon,\zeta} \leftarrow \sum_{i \in O} \sum_{j \in O} \sum_{k \in O} \sum_{l \in O} \sum_{a \in V} \sum_{b \in V} \sum_{c \in V} \sum_{d \in V} \frac{1}{2} \quad (7091)$$

$$\begin{aligned} & {}^1T_{c,i} \quad {}^1T_{d,k} \quad Y^{1,*}_{a,\epsilon} \quad Y^{2,*}_{i,\epsilon} \quad Y^{3,*}_{b,\zeta} \\ & Y^{4,*}_{j,\zeta} \quad {}^2D^{a,i,b,j} \quad {}^2T_{b,j,a,l} \quad V_{k,c,l,d} \end{aligned}$$

Factorized expression

$$\tau^0_{\gamma,\delta,w} = \sum_{a \in V} {}^2D^3_{a,w} Y^1_{a,\gamma} Y^{3,*}_{a,\delta} \quad (3r_D r_T^2 N_v) \quad (7092)$$

$$\tau^1_{\gamma,\delta,w} = \sum_{i \in O} {}^2D^4_{i,w} Y^2_{i,\gamma} Y^{4,*}_{i,\delta} \quad (3r_D r_T^2 N_o) \quad (7093)$$

$$\tau^2_{\gamma,\delta,w} = \sum_{\epsilon \in A} Z_{\epsilon,\gamma} \tau^0_{\epsilon,\delta,w} \tau^1_{\epsilon,\delta,w} \quad (3r_D r_T^3) \quad (7094)$$

$$\tau^3_{\gamma,\delta,w} = \sum_{i \in O} {}^2D^2_{i,w} Y^4_{i,\gamma} Y^{2,*}_{i,\delta} \quad (3r_D r_T^2 N_o) \quad (7095)$$

$$\tau^4_{\gamma,w,i} = \sum_{a \in V} {}^2D^1_{a,w} {}^1T_{a,i} Y^{1,*}_{a,\gamma} \quad (3r_D r_T N_o N_v) \quad (7096)$$

$$\tau^5_{\alpha,i} = \sum_{a \in V} {}^1T_{a,i} W^2_{a,\alpha} \quad (2r_V N_o N_v) \quad (7097)$$

$$\tau^6_{\alpha,\beta} = \sum_{i \in O} W^3_{i,\beta} \tau^5_{\alpha,i} \quad (2r_V^2 N_o) \quad (7098)$$

$$\tau^7_{\alpha,i} = \sum_{\beta \in B} W^1_{i,\beta} X_{\beta,\alpha} \tau^6_{\beta,\alpha} \quad (3r_V^2 N_o) \quad (7099)$$

$$\tau^8_{i,a} = \sum_{\alpha \in B} W^4_{a,\alpha} \tau^7_{\alpha,i} \quad (2r_V N_o N_v) \quad (7100)$$

$$\tau^9_{\gamma,i} = \sum_{a \in V} Y^3_{a,\gamma} \tau^8_{i,a} \quad (2r_T N_o N_v) \quad (7101)$$

$$\tau^{10}_{\gamma,\delta,w} = \sum_{i \in O} \tau^9_{\gamma,i} \tau^4_{\delta,w,i} \quad (2r_D r_T^2 N_o) \quad (7102)$$

$${}^2R^z_{\gamma,\delta} \leftarrow \sum_{\epsilon \in A} \sum_{w \in D} \frac{1}{2} \tau^{10}_{\epsilon,\gamma,w} \tau^2_{\epsilon,\delta,w} \tau^3_{\epsilon,\gamma,w} \quad (3r_D r_T^3) \quad (7103)$$

Raw expression

$${}^2R^z_{\epsilon,\zeta} \leftarrow \sum_{i \in O} \sum_{j \in O} \sum_{k \in O} \sum_{l \in O} \sum_{a \in V} \sum_{b \in V} \sum_{c \in V} \sum_{d \in V} \frac{1}{2} \quad (7104)$$

$$\begin{aligned} & {}^1T_{c,j} \quad {}^1T_{d,i} \quad Y^{1,*}_{a,\epsilon} \quad Y^{2,*}_{i,\epsilon} \quad Y^{3,*}_{b,\zeta} \\ & Y^{4,*}_{j,\zeta} \quad {}^2D^{a,i,b,j} \quad {}^2T_{b,k,a,l} \quad V_{k,c,l,d} \end{aligned}$$

Factorized expression

$$\tau^0_{\gamma,\delta,w} = \sum_{a \in V} {}^2D^3_{a,w} Y^3_{a,\gamma} Y^{3,*}_{a,\delta} \quad (3r_D r_T^2 N_v) \quad (7105)$$

$$\tau^1_{\gamma,\delta,w} = \sum_{i \in O} {}^2D^4_{i,w} Y^4_{i,\gamma} Y^{4,*}_{i,\delta} \quad (3r_D r_T^2 N_o) \quad (7106)$$

$$\tau^2_{\gamma,\delta,w} = \sum_{i \in O} {}^2D^2_{i,w} Y^2_{i,\gamma} Y^{2,*}_{i,\delta} \quad (3r_D r_T^2 N_o) \quad (7107)$$

$$\tau^3_{\gamma,w,i} = \sum_{a \in V} {}^2D^1_{a,w} {}^1T_{a,i} Y^{1,*}_{a,\gamma} \quad (3r_D r_T N_o N_v) \quad (7108)$$

$$\tau^4_{\alpha,i} = \sum_{a \in V} {}^1T_{a,i} W^2_{a,\alpha} \quad (2r_V N_o N_v) \quad (7109)$$

$$\tau^5_{\alpha,\beta} = \sum_{i \in O} W^3_{i,\beta} \tau^4_{\alpha,i} \quad (2r_V^2 N_o) \quad (7110)$$

$$\tau^6_{\alpha,i} = \sum_{\beta \in B} W^1_{i,\beta} X_{\beta,\alpha} \tau^5_{\beta,\alpha} \quad (3r_V^2 N_o) \quad (7111)$$

$$\tau^7_{i,a} = \sum_{\alpha \in B} W^4_{a,\alpha} \tau^6_{\alpha,i} \quad (2r_V N_o N_v) \quad (7112)$$

$$\tau^8_{\gamma,i} = \sum_{a \in V} Y^1_{a,\gamma} \tau^7_{i,a} \quad (2r_T N_o N_v) \quad (7113)$$

$$\tau^9_{\gamma,\delta,w} = \sum_{i \in O} \tau^8_{\gamma,i} \tau^3_{\delta,w,i} \quad (2r_D r_T^2 N_o) \quad (7114)$$

$$\tau^{10}_{\gamma,\delta,w} = \sum_{\epsilon \in A} Z_{\epsilon,\gamma} \tau^2_{\epsilon,\delta,w} \tau^9_{\epsilon,\delta,w} \quad (3r_D r_T^3) \quad (7115)$$

$${}^2R^z_{\gamma,\delta} \leftarrow \sum_{\epsilon \in A} \sum_{w \in D} \frac{1}{2} \tau^0_{\epsilon,\delta,w} \tau^1_{\epsilon,\delta,w} \tau^{10}_{\epsilon,\gamma,w} \quad (3r_D r_T^3) \quad (7116)$$

Raw expression

$${}^2R^z_{\epsilon,\zeta} \leftarrow \sum_{i \in O} \sum_{j \in O} \sum_{k \in O} \sum_{l \in O} \sum_{a \in V} \sum_{b \in V} \sum_{c \in V} \sum_{d \in V} \frac{1}{2} \quad (7117)$$

$$\begin{aligned} & {}^1T_{c,j} \quad {}^1T_{d,k} \quad Y^{1,*}_{a,\epsilon} \quad Y^{2,*}_{i,\epsilon} \quad Y^{3,*}_{b,\zeta} \\ & Y^{4,*}_{j,\zeta} \quad {}^2D^{a,i,b,j} \quad {}^2T_{a,i,b,l} \quad V_{k,c,l,d} \end{aligned}$$

Factorized expression

$$\tau^0_{\gamma,w,i} = \sum_{a \in V} {}^2D^3_{a,w} {}^1T_{a,i} Y^{3,*}_{a,\gamma} \quad (3r_D r_T N_o N_v) \quad (7118)$$

$$\tau^1_{\gamma,\alpha} = \sum_{a \in V} W^2_{a,\alpha} Y^3_{a,\gamma} \quad (2r_T r_V N_v) \quad (7119)$$

$$\tau^2_{\gamma,\alpha,i} = \sum_{\delta \in A} Z_{\gamma,\delta} Y^4_{i,\delta} \tau^1_{\delta,\alpha} \quad (3r_T^2 r_V N_o) \quad (7120)$$

$$\tau^3_{\gamma,\delta,w} = \sum_{a \in V} {}^2D^1_{a,w} Y^1_{a,\gamma} Y^{1,*}_{a,\delta} \quad (3r_D r_T^2 N_v) \quad (7121)$$

$$\tau^4_{\alpha,i} = \sum_{a \in V} {}^1T_{a,i} W^4_{a,\alpha} \quad (2r_V N_o N_v) \quad (7122)$$

$$\tau^5_{\alpha,i,j} = \sum_{\beta \in B} X_{\alpha,\beta} W^3_{j,\beta} \tau^4_{\beta,i} \quad (3r_V^2 N_o^2) \quad (7123)$$

$$\tau^6_{\gamma,\alpha,i} = \sum_{j \in O} Y^2_{j,\gamma} \tau^5_{\alpha,i,j} \quad (2r_T r_V N_o^2) \quad (7124)$$

$$\tau^7_{\gamma,\delta,\alpha,w} = \sum_{i \in O} {}^2D^2_{i,w} Y^{2,*}_{i,\delta} \tau^3_{\gamma,\delta,w} \tau^6_{\gamma,\alpha,i} \quad (4r_D r_T^2 r_V N_o) \quad (7125)$$

$$\tau^8_{\gamma,\alpha,w,i} = \sum_{\delta \in A} \tau^2_{\delta,\alpha,i} \tau^7_{\delta,\gamma,\alpha,w} \quad (2r_D r_T^2 r_V N_o) \quad (7126)$$

$$\tau^9_{\gamma,w,i,j} = \sum_{\alpha \in B} W^1_{i,\alpha} \tau^8_{\gamma,\alpha,w,j} \quad (2r_D r_T r_V N_o^2) \quad (7127)$$



$${}^2R^z_{\gamma,\delta} \leftarrow \sum_{w \in D} \sum_{i \in O} \sum_{j \in O} \frac{1}{2} {}^2D^4_{i,w} Y^{4,*}_{i,\delta} \tau^0_{\delta,w,j} \tau^9_{\gamma,w,j,i} \quad (4r_D r_T {}^2N_o^2) \quad (7128)$$

$${}^2R^z_{\sigma\gamma,\delta} \leftarrow \sum_{w \in D} \sum_{i \in O} \sum_{j \in O} \frac{1}{2} {}^2D^4_{i,w} Y^{4,*}_{i,\delta} \tau^0_{\delta,w,j} \tau^9_{\gamma,w,j,i} \quad (4r_D r_T {}^2N_o^2) \quad (7140)$$

Raw expression

$${}^2R^z_{\epsilon,\zeta} \leftarrow \sum_{i \in O} \sum_{j \in O} \sum_{k \in O} \sum_{l \in O} \sum_{a \in V} \sum_{b \in V} \sum_{c \in V} \sum_{d \in V} \frac{1}{2} \quad (7129)$$

$${}^1T_{c,j} \quad {}^1T_{d,k} \quad Y^{1,*}_{a,\epsilon} \quad Y^{2,*}_{i,\epsilon} \quad Y^{3,*}_{b,\zeta} \quad Y^{4,*}_{j,\zeta} \quad {}^2D^{a,i,b,j} \quad {}^2T_{b,l,a,i} \quad V_{k,c,l,d}$$

Factorized expression

$$\tau^0_{\gamma,w,i} = \sum_{a \in V} {}^2D^3_{a,w} {}^1T_{a,i} Y^{3,*}_{a,\gamma} \quad (3r_D r_T N_o N_v) \quad (7130)$$

$$\tau^1_{\gamma,\alpha} = \sum_{a \in V} W^2_{a,\alpha} Y^1_{a,\gamma} \quad (2r_T r_V N_v) \quad (7131)$$

$$\tau^2_{\gamma,\alpha,i} = \sum_{\delta \in A} Y^2_{i,\delta} Z_{\delta,\gamma} \tau^1_{\delta,\alpha} \quad (3r_T^2 r_V N_o) \quad (7132)$$

$$\tau^3_{\gamma,\delta,w} = \sum_{a \in V} {}^2D^1_{a,w} Y^3_{a,\gamma} Y^{1,*}_{a,\delta} \quad (3r_D r_T^2 N_v) \quad (7133)$$

$$\tau^4_{\alpha,i} = \sum_{a \in V} {}^1T_{a,i} W^4_{a,\alpha} \quad (2r_V N_o N_v) \quad (7134)$$

$$\tau^5_{\alpha,i,j} = \sum_{\beta \in B} X_{\alpha,\beta} W^3_{j,\beta} \tau^4_{\beta,i} \quad (3r_V^2 N_o^2) \quad (7135)$$

$$\tau^6_{\gamma,\alpha,i} = \sum_{j \in O} Y^4_{j,\gamma} \tau^5_{\alpha,i,j} \quad (2r_T r_V N_o^2) \quad (7136)$$

$$\tau^7_{\gamma,\delta,\alpha,w} = \sum_{i \in O} {}^2D^2_{i,w} Y^{2,*}_{i,\delta} \tau^3_{\gamma,\delta,w} \tau^6_{\gamma,\alpha,i} \quad (4r_D r_T^2 r_V N_o) \quad (7137)$$

$$\tau^8_{\gamma,\alpha,w,i} = \sum_{\delta \in A} \tau^2_{\delta,\alpha,i} \tau^7_{\delta,\gamma,\alpha,w} \quad (2r_D r_T^2 r_V N_o) \quad (7138)$$

$$\tau^9_{\gamma,w,i,j} = \sum_{\alpha \in B} W^1_{i,\alpha} \tau^8_{\gamma,\alpha,w,j} \quad (2r_D r_T r_V N_o^2) \quad (7139)$$

Raw expression

$${}^2R^z_{\epsilon,\zeta} \leftarrow - \sum_{i \in O} \sum_{j \in O} \sum_{k \in O} \sum_{l \in O} \sum_{a \in V} \sum_{b \in V} \sum_{c \in V} \sum_{d \in V} {}^1T_{a,k} \quad (7141)$$

$${}^1T_{c,i} \quad Y^{1,*}_{a,\epsilon} \quad Y^{2,*}_{i,\epsilon} \quad Y^{3,*}_{b,\zeta} \quad Y^{4,*}_{j,\zeta} \quad {}^2D^{a,i,b,j} \quad {}^2T_{b,j,d,l} \quad V_{k,c,l,d}$$

Factorized expression

$$\tau^0_{\alpha,i} = \sum_{a \in V} {}^1T_{a,i} W^2_{a,\alpha} \quad (2r_V N_o N_v) \quad (7142)$$

$$\tau^1_{\gamma,\alpha,w} = \sum_{i \in O} {}^2D^4_{i,w} Y^{4,*}_{i,\gamma} \tau^0_{\alpha,i} \quad (3r_D r_T r_V N_o) \quad (7143)$$

$$\tau^2_{\gamma,w,i} = \sum_{a \in V} {}^2D^3_{a,w} {}^1T_{a,i} Y^{3,*}_{a,\gamma} \quad (3r_D r_T N_o N_v) \quad (7144)$$

$$\tau^3_{\gamma,\alpha,w} = \sum_{i \in O} W^1_{i,\alpha} \tau^2_{\gamma,w,i} \quad (2r_D r_T r_V N_o) \quad (7145)$$

$$\tau^4_{\gamma,\delta,w} = \sum_{a \in V} {}^2D^1_{a,w} Y^1_{a,\gamma} Y^{1,*}_{a,\delta} \quad (3r_D r_T^2 N_v) \quad (7146)$$

$$\tau^5_{\gamma,\alpha} = \sum_{i \in O} W^3_{i,\alpha} Y^2_{i,\gamma} \quad (2r_T r_V N_o) \quad (7147)$$

$$\tau^6_{\gamma,\alpha} = \sum_{a \in V} W^4_{a,\alpha} Y^3_{a,\gamma} \quad (2r_T r_V N_v) \quad (7148)$$

$$\tau^7_{\gamma,\alpha,i} = \sum_{\delta \in A} Z_{\gamma,\delta} Y^4_{i,\delta} \tau^6_{\delta,\alpha} \quad (3r_T^2 r_V N_o) \quad (7149)$$

$$\tau^8_{\gamma,\alpha,w} = \sum_{\delta \in A} \sum_{i \in O} {}^2D^2_{i,w} Y^{2,*}_{i,\gamma} \tau^5_{\delta,\alpha} \tau^4_{\delta,\gamma,w} \tau^7_{\delta,\alpha,i} \quad (5r_D r_T^2 r_V N_o) \quad (7150)$$

$$\tau^9_{\gamma,\alpha,w} = \sum_{\beta \in B} X_{\alpha,\beta} \tau^8_{\gamma,\beta,w} \quad (2r_D r_T r_V^2) \quad (7151)$$

$${}^2R^z_{\gamma,\delta} \leftarrow \sum_{\alpha \in B} \sum_{w \in D} \frac{1}{2} \tau^1_{\delta,\alpha,w} \tau^3_{\delta,\alpha,w} \tau^9_{\gamma,\alpha,w} \quad (3r_D r_T^2 r_V) \quad (7152)$$

Raw expression

$${}^2R^z_{\epsilon,\zeta} \leftarrow - \sum_{i \in O} \sum_{j \in O} \sum_{k \in O} \sum_{l \in O} \sum_{a \in V} \sum_{b \in V} \sum_{c \in V} \sum_{d \in V} {}^1T_{a,k} \\ {}^1T_{c,i} Y^{1,*}_{a,\epsilon} Y^{2,*}_{i,\epsilon} Y^{3,*}_{b,\zeta} \\ Y^{4,*}_{j,\zeta} {}^2D^{a,i,b,j} {}^2T_{d,l,b,j} V_{k,c,l,d} \quad (7153)$$

Factorized expression

$$\tau^0_{\alpha,i} = \sum_{a \in V} {}^1T_{a,i} W^2_{a,\alpha} \quad (2r_V N_o N_v) \quad (7154)$$

$$\tau^1_{\gamma,\alpha,w} = \sum_{i \in O} {}^2D^4_{i,w} Y^{4,*}_{i,\gamma} \tau^0_{\alpha,i} \quad (3r_D r_T r_V N_o) \quad (7155)$$

$$\tau^2_{\gamma,w,i} = \sum_{a \in V} {}^2D^3_{a,w} {}^1T_{a,i} Y^{3,*}_{a,\gamma} \quad (3r_D r_T N_o N_v) \quad (7156)$$

$$\tau^3_{\gamma,\alpha,w} = \sum_{i \in O} W^1_{i,\alpha} \tau^2_{\gamma,w,i} \quad (2r_D r_T r_V N_o) \quad (7157)$$

$$\tau^4_{\gamma,\delta,w} = \sum_{a \in V} {}^2D^1_{a,w} Y^3_{a,\gamma} Y^{1,*}_{a,\delta} \quad (3r_D r_T^2 N_v) \quad (7158)$$

$$\tau^5_{\gamma,\alpha} = \sum_{a \in V} W^4_{a,\alpha} Y^1_{a,\gamma} \quad (2r_T r_V N_v) \quad (7159)$$

$$\tau^6_{\gamma,\alpha,i} = \sum_{\delta \in A} Y^2_{i,\delta} Z_{\delta,\gamma} \tau^5_{\delta,\alpha} \quad (3r_T^2 r_V N_o) \quad (7160)$$

$$\tau^7_{\gamma,\alpha} = \sum_{i \in O} W^3_{i,\alpha} Y^4_{i,\gamma} \quad (2r_T r_V N_o) \quad (7161)$$

$$\tau^8_{\gamma,\alpha,w} = \sum_{\delta \in A} \sum_{i \in O} {}^2D^2_{i,w} Y^{2,*}_{i,\gamma} \tau^7_{\delta,\alpha} \tau^4_{\delta,\gamma,w} \tau^6_{\delta,\alpha,i} \quad (5r_D r_T^2 r_V N_o) \quad (7162)$$

$$\tau^9_{\gamma,\alpha,w} = \sum_{\beta \in B} X_{\alpha,\beta} \tau^8_{\gamma,\beta,w} \quad (2r_D r_T r_V^2) \quad (7163)$$

$${}^2R^z_{\gamma,\delta} \leftarrow \sum_{\alpha \in B} \sum_{w \in D} \frac{1}{2} \tau^1_{\delta,\alpha,w} \tau^3_{\delta,\alpha,w} \tau^9_{\gamma,\alpha,w} \quad (3r_D r_T^2 r_V) \quad (7164)$$

Raw expression

$${}^2R^z_{\epsilon,\zeta} \leftarrow - \sum_{i \in O} \sum_{j \in O} \sum_{k \in O} \sum_{l \in O} \sum_{a \in V} \sum_{b \in V} \sum_{c \in V} \sum_{d \in V} {}^1T_{a,k} \\ {}^1T_{c,l} Y^{1,*}_{a,\epsilon} Y^{2,*}_{i,\epsilon} Y^{3,*}_{b,\zeta} \\ Y^{4,*}_{j,\zeta} {}^2D^{a,i,b,j} {}^2T_{b,j,d,i} V_{k,d,l,c} \quad (7165)$$

Factorized expression

$$\tau^0_{\gamma,w,i} = \sum_{a \in V} {}^2D^3_{a,w} {}^1T_{a,i} Y^{3,*}_{a,\gamma} \quad (3r_D r_T N_o N_v) \quad (7166)$$

$$\tau^1_{\gamma,\alpha} = \sum_{a \in V} W^2_{a,\alpha} Y^3_{a,\gamma} \quad (2r_T r_V N_v) \quad (7167)$$

$$\tau^2_{\alpha,i} = \sum_{a \in V} {}^1T_{a,i} W^4_{a,\alpha} \quad (2r_V N_o N_v) \quad (7168)$$

$$\tau^3_{\alpha,i,j} = \sum_{\beta \in B} X_{\alpha,\beta} W^3_{j,\beta} \tau^2_{\beta,i} \quad (3r_V^2 N_o^2) \quad (7169)$$

$$\tau^4_{\gamma,\alpha,i} = \sum_{j \in O} Y^4_{j,\gamma} \tau^3_{\alpha,i,j} \quad (2r_T r_V N_o^2) \quad (7170)$$

$$\tau^5_{\gamma,i,j} = \sum_{\alpha \in B} W^1_{j,\alpha} \tau^1_{\gamma,\alpha} \tau^4_{\gamma,\alpha,i} \quad (3r_T r_V N_o^2) \quad (7171)$$

$$\tau^6_{\gamma,i,j} = \sum_{\delta \in A} Z_{\gamma,\delta} \tau^5_{\delta,i,j} \quad (2r_T^2 N_o^2) \quad (7172)$$

$$\tau^7_{\gamma,\delta,w} = \sum_{i \in O} \sum_{j \in O} {}^2D^4_{i,w} Y^{4,*}_{i,\delta} \tau^0_{\delta,w,j} \tau^6_{\gamma,i,j} \quad (4r_D r_T^2 N_o^2) \quad (7173)$$

$$\tau^8_{\gamma,\delta,w} = \sum_{a \in V} {}^2D^1_{a,w} Y^1_{a,\gamma} Y^{1,*}_{a,\delta} \quad (3r_D r_T^2 N_v) \quad (7174)$$

$$\tau^9_{\gamma,\delta,w} = \sum_{i \in O} {}^2D^2_{i,w} Y^2_{i,\gamma} Y^{2,*}_{i,\delta} \quad (3r_D r_T^2 N_o) \quad (7175)$$

$${}^2R^z_{\gamma,\delta} \leftarrow \sum_{\epsilon \in A} \sum_{w \in D} \frac{1}{2} \tau^7_{\epsilon,\delta,w} \tau^8_{\epsilon,\gamma,w} \tau^9_{\epsilon,\gamma,w} \quad (3r_D r_T^3) \quad (7176)$$

Raw expression

$${}^2R^z_{\epsilon,\zeta} \leftarrow - \sum_{i \in O} \sum_{j \in O} \sum_{k \in O} \sum_{l \in O} \sum_{a \in V} \sum_{b \in V} \sum_{c \in V} \sum_{d \in V} {}^1T_{a,k} \\ {}^1T_{c,l} Y^{1,*}_{a,\epsilon} Y^{2,*}_{i,\epsilon} Y^{3,*}_{b,\zeta} \\ Y^{4,*}_{j,\zeta} {}^2D^{a,i,b,j} {}^2T_{d,i,b,j} V_{k,d,l,c} \quad (7177)$$

Factorized expression

$$\tau^0_{\gamma,w,i} = \sum_{a \in V} {}^2D^3_{a,w} {}^1T_{a,i} Y^{3,*}_{a,\gamma} \quad (3r_D r_T N_o N_v) \quad (7178)$$

$$\tau^1_{\gamma,\alpha} = \sum_{a \in V} W^2_{a,\alpha} Y^1_{a,\gamma} \quad (2r_T r_V N_v) \quad (7179)$$

$$\tau^2_{\alpha,i} = \sum_{a \in V} {}^1T_{a,i} W^4_{a,\alpha} \quad (2r_V N_o N_v) \quad (7180)$$

$$\tau^3_{\alpha,i,j} = \sum_{\beta \in B} X_{\alpha,\beta} W^3_{j,\beta} \tau^2_{\beta,i} \quad (3r_V^2 N_o^2) \quad (7181)$$

$$\tau^4_{\gamma,\alpha,i} = \sum_{j \in O} Y^2_{j,\gamma} \tau^3_{\alpha,i,j} \quad (2r_T r_V N_o^2) \quad (7182)$$

$$\tau^5_{\gamma,i,j} = \sum_{\alpha \in B} W^1_{j,\alpha} \tau^1_{\gamma,\alpha} \tau^4_{\gamma,\alpha,i} \quad (3r_T r_V N_o^2) \quad (7183)$$

$$\tau^6_{\gamma,i,j} = \sum_{\delta \in A} Z_{\delta,\gamma} \tau^5_{\delta,i,j} \quad (2r_T^2 N_o^2) \quad (7184)$$

$$\tau^7_{\gamma,\delta,w} = \sum_{i \in O} \sum_{j \in O} {}^2D^4_{i,w} Y^{4,*}_{i,\delta} \tau^0_{\delta,w,j} \tau^6_{\gamma,i,j} \quad (4r_D r_T^2 N_o^2) \quad (7185)$$

$$\tau^8_{\gamma,\delta,w} = \sum_{a \in V} {}^2D^1_{a,w} Y^3_{a,\gamma} Y^{1,*}_{a,\delta} \quad (3r_D r_T^2 N_v) \quad (7186)$$

$$\tau^9_{\gamma,\delta,w} = \sum_{i \in O} {}^2D^2_{i,w} Y^4_{i,\gamma} Y^{2,*}_{i,\delta} \quad (3r_D r_T^2 N_o) \quad (7187)$$

$${}^2R^z_{\gamma,\delta} \leftarrow \sum_{\epsilon \in A} \sum_{w \in D} \frac{1}{2} \tau^7_{\epsilon,\delta,w} \tau^8_{\epsilon,\gamma,w} \tau^9_{\epsilon,\gamma,w} \quad (3r_D r_T^3) \quad (7188)$$

Raw expression

$${}^2R^z_{\epsilon,\zeta} \leftarrow - \sum_{i \in O} \sum_{j \in O} \sum_{k \in O} \sum_{l \in O} \sum_{a \in V} \sum_{b \in V} \sum_{c \in V} \sum_{d \in V} {}^1T_{b,k} \\ {}^1T_{c,j} Y^{1,*}_{a,\epsilon} Y^{2,*}_{i,\epsilon} Y^{3,*}_{b,\zeta} \\ Y^{4,*}_{j,\zeta} {}^2D^{a,i,b,j} {}^2T_{a,i,d,l} V_{k,c,l,d} \quad (7189)$$

Factorized expression

$$\tau^0_{\gamma,\delta,w} = \sum_{i \in O} {}^2D^4_{i,w} Y^4_{i,\gamma} Y^{4,*}_{i,\delta} \quad (3r_D r_T^2 N_o) \quad (7190)$$

$$\tau^1_{\gamma,w,i} = \sum_{a \in V} {}^2D^3_{a,w} {}^1T_{a,i} Y^{3,*}_{a,\gamma} \quad (3r_D r_T N_o N_v) \quad (7191)$$

$$\tau^2_{\alpha,i} = \sum_{a \in V} {}^1T_{a,i} W^2_{a,\alpha} \quad (2r_V N_o N_v) \quad (7192)$$

$$\tau^3_{\alpha,\beta} = \sum_{i \in O} W^3_{i,\beta} \tau^2_{\alpha,i} \quad (2r_V^2 N_o) \quad (7193)$$

$$\tau^4_{\alpha,i} = \sum_{\beta \in B} W^1_{i,\beta} X_{\beta,\alpha} \tau^3_{\beta,\alpha} \quad (3r_V^2 N_o) \quad (7194)$$

$$\tau^5_{i,a} = \sum_{\alpha \in B} W^4_{a,\alpha} \tau^4_{\alpha,i} \quad (2r_V N_o N_v) \quad (7195)$$

$$\tau^6_{\gamma,i} = \sum_{a \in V} Y^3_{a,\gamma} \tau^5_{i,a} \quad (2r_T N_o N_v) \quad (7196)$$

$$\tau^7_{\gamma,\delta,w} = \sum_{i \in O} \tau^6_{\gamma,i} \tau^1_{\delta,w,i} \quad (2r_D r_T^2 N_o) \quad (7197)$$

$$\tau^8_{\gamma,\delta,w} = \sum_{a \in V} {}^2D^1_{a,w} Y^1_{a,\gamma} Y^{1,*}_{a,\delta} \quad (3r_D r_T^2 N_v) \quad (7198)$$

$$\tau^9_{\gamma,\delta,w} = \sum_{i \in O} {}^2D^2_{i,w} Y^2_{i,\gamma} Y^{2,*}_{i,\delta} \quad (3r_D r_T^2 N_o) \quad (7199)$$

$$\tau^{10}_{\gamma,\delta,w} = \sum_{\epsilon \in A} Z_{\epsilon,\gamma} \tau^8_{\epsilon,\delta,w} \tau^9_{\epsilon,\delta,w} \quad (3r_D r_T^3) \quad (7200)$$

$${}^2R^z_{\gamma,\delta} \leftarrow \sum_{\epsilon \in A} \sum_{w \in D} \frac{1}{2} \tau^0_{\epsilon,\delta,w} \tau^{10}_{\epsilon,\gamma,w} \tau^7_{\epsilon,\delta,w} \quad (3r_D r_T^3) \quad (7201)$$

Raw expression

$${}^2R^z_{\epsilon,\zeta} \leftarrow - \sum_{i \in O} \sum_{j \in O} \sum_{k \in O} \sum_{l \in O} \sum_{a \in V} \sum_{b \in V} \sum_{c \in V} \sum_{d \in V} {}^1T_{b,k} \\ {}^1T_{c,j} \ Y^{1,*}_{a,\epsilon} \ Y^{2,*}_{i,\epsilon} \ Y^{3,*}_{b,\zeta} \\ Y^{4,*}_{j,\zeta} \ {}^2D^{a,i,b,j} \ {}^2T_{d,l,a,i} \ V_{k,c,l,d} \quad (7202)$$

Factorized expression

$$\tau^0_{\gamma,\delta,w} = \sum_{i \in O} {}^2D^4_{i,w} Y^2_{i,\gamma} Y^{4,*}_{i,\delta} \quad (3r_D r_T^2 N_o) \quad (7203)$$

$$\tau^1_{\gamma,w,i} = \sum_{a \in V} {}^2D^3_{a,w} {}^1T_{a,i} Y^{3,*}_{a,\gamma} \quad (3r_D r_T N_o N_v) \quad (7204)$$

$$\tau^2_{\alpha,i} = \sum_{a \in V} {}^1T_{a,i} W^2_{a,\alpha} \quad (2r_V N_o N_v) \quad (7205)$$

$$\tau^3_{\alpha,\beta} = \sum_{i \in O} W^3_{i,\beta} \tau^2_{\alpha,i} \quad (2r_V^2 N_o) \quad (7206)$$

$$\tau^4_{\alpha,i} = \sum_{\beta \in B} W^1_{i,\beta} X_{\beta,\alpha} \tau^3_{\beta,\alpha} \quad (3r_V^2 N_o) \quad (7207)$$

$$\tau^5_{i,a} = \sum_{\alpha \in B} W^4_{a,\alpha} \tau^4_{\alpha,i} \quad (2r_V N_o N_v) \quad (7208)$$

$$\tau^6_{\gamma,i} = \sum_{a \in V} Y^1_{a,\gamma} \tau^5_{i,a} \quad (2r_T N_o N_v) \quad (7209)$$

$$\tau^7_{\gamma,\delta,w} = \sum_{i \in O} \tau^6_{\gamma,i} \tau^1_{\delta,w,i} \quad (2r_D r_T^2 N_o) \quad (7210)$$

$$\tau^8_{\gamma,\delta,w} = \sum_{\epsilon \in A} Z_{\epsilon,\gamma} \tau^0_{\epsilon,\delta,w} \tau^7_{\epsilon,\delta,w} \quad (3r_D r_T^3) \quad (7211)$$

$$\tau^9_{\gamma,\delta,w} = \sum_{a \in V} {}^2D^1_{a,w} Y^3_{a,\gamma} Y^{1,*}_{a,\delta} \quad (3r_D r_T^2 N_v) \quad (7212)$$

$$\tau^{10}_{\gamma,\delta,w} = \sum_{i \in O} {}^2D^2_{i,w} Y^4_{i,\gamma} Y^{2,*}_{i,\delta} \quad (3r_D r_T^2 N_o) \quad (7213)$$

$${}^2R^z_{\gamma,\delta} \leftarrow \sum_{\epsilon \in A} \sum_{w \in D} \frac{1}{2} \tau^{10}_{\epsilon,\gamma,w} \tau^8_{\epsilon,\delta,w} \tau^9_{\epsilon,\gamma,w} \quad (3r_D r_T^3) \quad (7214)$$

Raw expression

$${}^2R^z_{\epsilon,\zeta} \leftarrow - \sum_{i \in O} \sum_{j \in O} \sum_{k \in O} \sum_{l \in O} \sum_{a \in V} \sum_{b \in V} \sum_{c \in V} \sum_{d \in V} {}^1T_{b,k} \\ {}^1T_{c,l} \ Y^{1,*}_{a,\epsilon} \ Y^{2,*}_{i,\epsilon} \ Y^{3,*}_{b,\zeta} \\ Y^{4,*}_{j,\zeta} \ {}^2D^{a,i,b,j} \ {}^2T_{a,i,d,j} \ V_{k,d,l,c} \quad (7215)$$

Factorized expression

$$\tau^0_{\gamma,\delta,w} = \sum_{a \in V} {}^2D^1_{a,w} Y^1_{a,\gamma} Y^{1,*}_{a,\delta} \quad (3r_D r_T^2 N_v) \quad (7216)$$

$$\tau^1_{\alpha,i} = \sum_{a \in V} {}^1T_{a,i} W^4_{a,\alpha} \quad (2r_V N_o N_v) \quad (7217)$$

$$\tau^2_{\gamma,\alpha,w} = \sum_{i \in O} {}^2D^4_{i,w} Y^{4,*}_{i,\gamma} \tau^1_{\alpha,i} \quad (3r_D r_T r_V N_o) \quad (7218)$$

$$\tau^3_{\gamma,\delta,w} = \sum_{a \in V} {}^2D^3_{a,w} Y^3_{a,\gamma} Y^{3,*}_{a,\delta} \quad (3r_D r_T^2 N_v) \quad (7219)$$

$$\tau^4_{\gamma,\delta,w,i} = \sum_{\epsilon \in A} Z_{\gamma,\epsilon} Y^4_{i,\epsilon} \tau^3_{\epsilon,\delta,w} \quad (3r_D r_T^3 N_o) \quad (7220)$$

$$\tau^5_{\gamma,\delta,\alpha,w} = \sum_{i \in O} W^3_{i,\alpha} \tau^2_{\delta,\alpha,w} \tau^4_{\gamma,\delta,w,i} \quad (3r_D r_T^2 r_V N_o) \quad (7221)$$

$$\tau^6_{\alpha,i} = \sum_{a \in V} {}^1T_{a,i} W^2_{a,\alpha} \quad (2r_V N_o N_v) \quad (7222)$$

$$\tau^7_{\alpha,i,j} = \sum_{\beta \in B} W^1_{j,\beta} X_{\beta,\alpha} \tau^6_{\beta,i} \quad (3r_V^2 N_o^2) \quad (7223)$$

$$\tau^8_{\gamma,\alpha,i} = \sum_{j \in O} Y^2_{j,\gamma} \tau^7_{\alpha,i,j} \quad (2r_T r_V N_o^2) \quad (7224)$$

$$\tau^9_{\gamma,\delta,w,i} = \sum_{\alpha \in B} \tau^8_{\gamma,\alpha,i} \tau^5_{\gamma,\delta,\alpha,w} \quad (2r_D r_T^2 r_V N_o) \quad (7225)$$

$${}^2R^z_{\gamma,\delta} \leftarrow \sum_{\epsilon \in A} \sum_{w \in D} \sum_{i \in O} \frac{1}{2} {}^2D^2_{i,w} Y^{2,*}_{i,\gamma} \tau^0_{\epsilon,\gamma,w} \tau^9_{\epsilon,\delta,w,i} \quad (4r_D r_T^3 N_o) \quad (7226)$$

Raw expression

$${}^2R_{\epsilon,\zeta}^z \leftarrow - \sum_{i \in O} \sum_{j \in O} \sum_{k \in O} \sum_{l \in O} \sum_{a \in V} \sum_{b \in V} \sum_{c \in V} \sum_{d \in V} {}^1T_{b,k} \\ {}^1T_{c,l} Y^{1,*}_{a,\epsilon} Y^{2,*}_{i,\epsilon} Y^{3,*}_{b,\zeta} Y^{4,*}_{j,\zeta} {}^2D^{a,i,b,j} {}^2T_{d,j,a,i} V_{k,d,l,c} \quad (7227)$$

Factorized expression

$$\tau^0_{\gamma,\delta,w} = \sum_{a \in V} {}^2D^1_{a,w} Y^3_{a,\gamma} Y^{1,*}_{a,\delta} (3r_D r_T^2 N_v) \quad (7228)$$

$$\tau^1_{\alpha,i} = \sum_{a \in V} {}^1T_{a,i} W^2_{a,\alpha} (2r_V N_o N_v) \quad (7229)$$

$$\tau^2_{\gamma,\alpha,w} = \sum_{i \in O} {}^2D^4_{i,w} Y^{4,*}_{i,\gamma} \tau^1_{\alpha,i} (3r_D r_T r_V N_o) \quad (7230)$$

$$\tau^3_{\gamma,\delta,w} = \sum_{a \in V} {}^2D^3_{a,w} Y^1_{a,\gamma} Y^{3,*}_{a,\delta} (3r_D r_T^2 N_v) \quad (7231)$$

$$\tau^4_{\gamma,\delta,w,i} = \sum_{\epsilon \in A} Y^2_{i,\epsilon} Z_{\epsilon,\gamma} \tau^3_{\epsilon,\delta,w} (3r_D r_T^3 N_o) \quad (7232)$$

$$\tau^5_{\gamma,\delta,\alpha,w} = \sum_{i \in O} W^1_{i,\alpha} \tau^2_{\delta,\alpha,w} \tau^4_{\gamma,\delta,w,i} (3r_D r_T^2 r_V N_o) \quad (7233)$$

$$\tau^6_{\alpha,i} = \sum_{a \in V} {}^1T_{a,i} W^4_{a,\alpha} (2r_V N_o N_v) \quad (7234)$$

$$\tau^7_{\alpha,i,j} = \sum_{\beta \in B} X_{\alpha,\beta} W^3_{j,\beta} \tau^6_{\beta,i} (3r_V^2 N_o^2) \quad (7235)$$

$$\tau^8_{\gamma,\alpha,i} = \sum_{j \in O} Y^4_{j,\gamma} \tau^7_{\alpha,i,j} (2r_T r_V N_o^2) \quad (7236)$$

$$\tau^9_{\gamma,\delta,w,i} = \sum_{\alpha \in B} \tau^8_{\gamma,\alpha,i} \tau^5_{\gamma,\delta,\alpha,w} (2r_D r_T^2 r_V N_o) \quad (7237)$$

$${}^2R_{\gamma,\delta}^z \leftarrow \sum_{\epsilon \in A} \sum_{w \in D} \sum_{i \in O} \frac{1}{2} {}^2D^2_{i,w} Y^{2,*}_{i,\gamma} \tau^0_{\epsilon,\gamma,w} \tau^9_{\epsilon,\delta,w,i} (4r_D r_T^3 N_o^2) \quad (7238)$$

Raw expression

$${}^2R_{\epsilon,\zeta}^z \leftarrow - \sum_{i \in O} \sum_{j \in O} \sum_{k \in O} \sum_{l \in O} \sum_{a \in V} \sum_{b \in V} \sum_{c \in V} \sum_{d \in V} {}^1T_{c,k} \\ {}^1T_{d,i} Y^{1,*}_{a,\epsilon} Y^{2,*}_{i,\epsilon} Y^{3,*}_{b,\zeta} Y^{4,*}_{j,\zeta} {}^2D^{a,i,b,j} {}^2T_{a,l,b,j} V_{k,c,l,d} \quad (7239)$$

Factorized expression

$$\tau^0_{\gamma,\delta,w} = \sum_{a \in V} {}^2D^3_{a,w} Y^3_{a,\gamma} Y^{3,*}_{a,\delta} (3r_D r_T^2 N_v) \quad (7240)$$

$$\tau^1_{\gamma,\delta,w} = \sum_{i \in O} {}^2D^4_{i,w} Y^4_{i,\gamma} Y^{4,*}_{i,\delta} (3r_D r_T^2 N_o) \quad (7241)$$

$$\tau^2_{\gamma,\delta,w} = \sum_{a \in V} {}^2D^1_{a,w} Y^1_{a,\gamma} Y^{1,*}_{a,\delta} (3r_D r_T^2 N_v) \quad (7242)$$

$$\tau^3_{\alpha,i} = \sum_{a \in V} {}^1T_{a,i} W^4_{a,\alpha} (2r_V N_o N_v) \quad (7243)$$

$$\tau^4_{\alpha,\beta} = \sum_{i \in O} W^1_{i,\alpha} \tau^3_{\beta,i} (2r_V^2 N_o) \quad (7244)$$

$$\tau^5_{\alpha,i} = \sum_{\beta \in B} X_{\alpha,\beta} W^3_{i,\beta} \tau^4_{\alpha,\beta} (3r_V^2 N_o) \quad (7245)$$

$$\tau^6_{i,a} = \sum_{\alpha \in B} W^2_{a,\alpha} \tau^5_{\alpha,i} (2r_V N_o N_v) \quad (7246)$$

$$\tau^7_{i,j} = \sum_{a \in V} {}^1T_{a,i} \tau^6_{j,a} (2N_o^2 N_v) \quad (7247)$$

$$\tau^8_{\gamma,i} = \sum_{j \in O} Y^2_{j,\gamma} \tau^7_{i,j} (2r_T N_o^2) \quad (7248)$$

$$\tau^9_{\gamma,\delta,w} = \sum_{i \in O} {}^2D^2_{i,w} Y^{2,*}_{i,\delta} \tau^8_{\gamma,i} (3r_D r_T^2 N_o) \quad (7249)$$

$$\tau^{10}_{\gamma,\delta,w} = \sum_{\epsilon \in A} Z_{\epsilon,\gamma} \tau^2_{\epsilon,\delta,w} \tau^9_{\epsilon,\delta,w} (3r_D r_T^3) \quad (7250)$$

$${}^2R_{\gamma,\delta}^z \leftarrow \sum_{\epsilon \in A} \sum_{w \in D} \frac{1}{2} \tau^0_{\epsilon,\delta,w} \tau^1_{\epsilon,\delta,w} \tau^{10}_{\epsilon,\gamma,w} (3r_D r_T^3) \quad (7251)$$

Raw expression

$${}^2R^z_{\epsilon,\zeta} \leftarrow - \sum_{i \in O} \sum_{j \in O} \sum_{k \in O} \sum_{l \in O} \sum_{a \in V} \sum_{b \in V} \sum_{c \in V} \sum_{d \in V} {}^1T_{c,k} \\ {}^1T_{d,i} Y^{1,*}_{a,\epsilon} Y^{2,*}_{i,\epsilon} Y^{3,*}_{b,\zeta} \\ Y^{4,*}_{j,\zeta} {}^2D^{a,i,b,j} {}^2T_{b,j,a,l} V_{k,c,l,d} \quad (7252)$$

Factorized expression

$$\tau^0_{\gamma,\delta,w} = \sum_{a \in V} {}^2D^3_{a,w} Y^1_{a,\gamma} Y^{3,*}_{a,\delta} (3r_D r_T^2 N_v) \quad (7253)$$

$$\tau^1_{\gamma,\delta,w} = \sum_{i \in O} {}^2D^4_{i,w} Y^2_{i,\gamma} Y^{4,*}_{i,\delta} (3r_D r_T^2 N_o) \quad (7254)$$

$$\tau^2_{\gamma,\delta,w} = \sum_{\epsilon \in A} Z_{\epsilon,\gamma} \tau^0_{\epsilon,\delta,w} \tau^1_{\epsilon,\delta,w} (3r_D r_T^3) \quad (7255)$$

$$\tau^3_{\gamma,\delta,w} = \sum_{a \in V} {}^2D^1_{a,w} Y^3_{a,\gamma} Y^{1,*}_{a,\delta} (3r_D r_T^2 N_v) \quad (7256)$$

$$\tau^4_{\alpha,i} = \sum_{a \in V} {}^1T_{a,i} W^4_{a,\alpha} (2r_V N_o N_v) \quad (7257)$$

$$\tau^5_{\alpha,\beta} = \sum_{i \in O} W^1_{i,\alpha} \tau^4_{\beta,i} (2r_V^2 N_o) \quad (7258)$$

$$\tau^6_{\alpha,i} = \sum_{\beta \in B} X_{\alpha,\beta} W^3_{i,\beta} \tau^5_{\alpha,\beta} (3r_V^2 N_o) \quad (7259)$$

$$\tau^7_{i,a} = \sum_{\alpha \in B} W^2_{a,\alpha} \tau^6_{\alpha,i} (2r_V N_o N_v) \quad (7260)$$

$$\tau^8_{i,j} = \sum_{a \in V} {}^1T_{a,i} \tau^7_{j,a} (2N_o^2 N_v) \quad (7261)$$

$$\tau^9_{\gamma,i} = \sum_{j \in O} Y^4_{j,\gamma} \tau^8_{i,j} (2r_T N_o^2) \quad (7262)$$

$$\tau^{10}_{\gamma,\delta,w} = \sum_{i \in O} {}^2D^2_{i,w} Y^{2,*}_{i,\delta} \tau^9_{\gamma,i} (3r_D r_T^2 N_o) \quad (7263)$$

$${}^2R^z_{\gamma,\delta} \leftarrow \sum_{\epsilon \in A} \sum_{w \in D} \frac{1}{2} \tau^{10}_{\epsilon,\gamma,w} \tau^2_{\epsilon,\delta,w} \tau^3_{\epsilon,\gamma,w} (3r_D r_T^3) \quad (7264)$$

Raw expression

$${}^2R^z_{\epsilon,\zeta} \leftarrow - \sum_{i \in O} \sum_{j \in O} \sum_{k \in O} \sum_{l \in O} \sum_{a \in V} \sum_{b \in V} \sum_{c \in V} \sum_{d \in V} {}^1T_{c,k} \\ {}^1T_{d,j} Y^{1,*}_{a,\epsilon} Y^{2,*}_{i,\epsilon} Y^{3,*}_{b,\zeta} \\ Y^{4,*}_{j,\zeta} {}^2D^{a,i,b,j} {}^2T_{a,i,b,l} V_{k,c,l,d} \quad (7265)$$

Factorized expression

$$\tau^0_{\gamma,\delta,w} = \sum_{a \in V} {}^2D^3_{a,w} Y^3_{a,\gamma} Y^{3,*}_{a,\delta} (3r_D r_T^2 N_v) \quad (7266)$$

$$\tau^1_{\alpha,i} = \sum_{a \in V} {}^1T_{a,i} W^4_{a,\alpha} (2r_V N_o N_v) \quad (7267)$$

$$\tau^2_{\alpha,\beta} = \sum_{i \in O} W^1_{i,\alpha} \tau^1_{\beta,i} (2r_V^2 N_o) \quad (7268)$$

$$\tau^3_{\alpha,i} = \sum_{\beta \in B} X_{\alpha,\beta} W^3_{i,\beta} \tau^2_{\alpha,\beta} (3r_V^2 N_o) \quad (7269)$$

$$\tau^4_{i,a} = \sum_{\alpha \in B} W^2_{a,\alpha} \tau^3_{\alpha,i} (2r_V N_o N_v) \quad (7270)$$

$$\tau^5_{i,j} = \sum_{a \in V} {}^1T_{a,i} \tau^4_{j,a} (2N_o^2 N_v) \quad (7271)$$

$$\tau^6_{\gamma,i} = \sum_{j \in O} Y^4_{j,\gamma} \tau^5_{i,j} (2r_T N_o^2) \quad (7272)$$

$$\tau^7_{\gamma,\delta,w} = \sum_{i \in O} {}^2D^4_{i,w} Y^{4,*}_{i,\delta} \tau^6_{\gamma,i} (3r_D r_T^2 N_o) \quad (7273)$$

$$\tau^8_{\gamma,\delta,w} = \sum_{a \in V} {}^2D^1_{a,w} Y^1_{a,\gamma} Y^{1,*}_{a,\delta} (3r_D r_T^2 N_v) \quad (7274)$$

$$\tau^9_{\gamma,\delta,w} = \sum_{i \in O} {}^2D^2_{i,w} Y^2_{i,\gamma} Y^{2,*}_{i,\delta} (3r_D r_T^2 N_o) \quad (7275)$$

$$\tau^{10}_{\gamma,\delta,w} = \sum_{\epsilon \in A} Z_{\epsilon,\gamma} \tau^8_{\epsilon,\delta,w} \tau^9_{\epsilon,\delta,w} (3r_D r_T^3) \quad (7276)$$

$${}^2R^z_{\gamma,\delta} \leftarrow \sum_{\epsilon \in A} \sum_{w \in D} \frac{1}{2} \tau^0_{\epsilon,\delta,w} \tau^{10}_{\epsilon,\gamma,w} \tau^7_{\epsilon,\delta,w} (3r_D r_T^3) \quad (7277)$$

Raw expression

$${}^2R^z_{\epsilon,\zeta} \leftarrow - \sum_{i \in O} \sum_{j \in O} \sum_{k \in O} \sum_{l \in O} \sum_{a \in V} \sum_{b \in V} \sum_{c \in V} \sum_{d \in V} {}^1T_{c,k} \\ {}^1T_{d,j} Y^{1,*}_{a,\epsilon} Y^{2,*}_{i,\epsilon} Y^{3,*}_{b,\zeta} \\ Y^{4,*}_{j,\zeta} {}^2D^{a,i,b,j} {}^2T_{b,l,a,i} V_{k,c,l,d} \quad (7278)$$

Factorized expression

$$\tau^0_{\gamma,\delta,w} = \sum_{a \in V} {}^2D^3_{a,w} Y^1_{a,\gamma} Y^{3,*}_{a,\delta} (3r_D r_T^2 N_v) \quad (7279)$$

$$\tau^1_{\alpha,i} = \sum_{a \in V} {}^1T_{a,i} W^4_{a,\alpha} (2r_V N_o N_v) \quad (7280)$$

$$\tau^2_{\alpha,\beta} = \sum_{i \in O} W^1_{i,\alpha} \tau^1_{\beta,i} (2r_V^2 N_o) \quad (7281)$$

$$\tau^3_{\alpha,i} = \sum_{\beta \in B} X_{\alpha,\beta} W^3_{i,\beta} \tau^2_{\alpha,\beta} (3r_V^2 N_o) \quad (7282)$$

$$\tau^4_{i,a} = \sum_{\alpha \in B} W^2_{a,\alpha} \tau^3_{\alpha,i} (2r_V N_o N_v) \quad (7283)$$

$$\tau^5_{i,j} = \sum_{a \in V} {}^1T_{a,i} \tau^4_{j,a} (2N_o^2 N_v) \quad (7284)$$

$$\tau^6_{\gamma,i} = \sum_{j \in O} Y^2_{j,\gamma} \tau^5_{i,j} (2r_T N_o^2) \quad (7285)$$

$$\tau^7_{\gamma,\delta,w} = \sum_{i \in O} {}^2D^4_{i,w} Y^{4,*}_{i,\delta} \tau^6_{\gamma,i} (3r_D r_T^2 N_o) \quad (7286)$$

$$\tau^8_{\gamma,\delta,w} = \sum_{\epsilon \in A} Z_{\epsilon,\gamma} \tau^0_{\epsilon,\delta,w} \tau^7_{\epsilon,\delta,w} (3r_D r_T^3) \quad (7287)$$

$$\tau^9_{\gamma,\delta,w} = \sum_{a \in V} {}^2D^1_{a,w} Y^3_{a,\gamma} Y^{1,*}_{a,\delta} (3r_D r_T^2 N_v) \quad (7288)$$

$$\tau^{10}_{\gamma,\delta,w} = \sum_{i \in O} {}^2D^2_{i,w} Y^4_{i,\gamma} Y^{2,*}_{i,\delta} (3r_D r_T^2 N_o) \quad (7289)$$

$${}^2R^z_{\gamma,\delta} \leftarrow \sum_{\epsilon \in A} \sum_{w \in D} \frac{1}{2} \tau^{10}_{\epsilon,\gamma,w} \tau^8_{\epsilon,\delta,w} \tau^9_{\epsilon,\gamma,w} (3r_D r_T^3) \quad (7290)$$

## I. Contributions from $(H^2 T^2 T)_c$

Raw expression

$${}^2R^z_{\epsilon,\zeta} \leftarrow \sum_{i \in O} \sum_{j \in O} \sum_{k \in O} \sum_{l \in O} \sum_{a \in V} \sum_{b \in V} \sum_{c \in V} \sum_{d \in V} Y^{1,*}_{a,\epsilon} Y^{2,*}_{i,\epsilon} \\ Y^{3,*}_{b,\zeta} Y^{4,*}_{j,\zeta} {}^2D^{a,i,b,j} {}^2T_{a,i,c,k} {}^2T_{b,j,d,l} V_{k,c,l,d} \quad (7291)$$

Factorized expression

$$\tau^0_{\gamma,\delta,w} = \sum_{a \in V} {}^2D^1_{a,w} Y^1_{a,\gamma} Y^{1,*}_{a,\delta} (3r_D r_T^2 N_v) \quad (7292)$$

$$\tau^1_{\gamma,\delta,w} = \sum_{i \in O} {}^2D^2_{i,w} Y^2_{i,\gamma} Y^{2,*}_{i,\delta} (3r_D r_T^2 N_o) \quad (7293)$$

$$\tau^2_{\gamma,\delta,w} = \sum_{a \in V} {}^2D^3_{a,w} Y^1_{a,\gamma} Y^{3,*}_{a,\delta} (3r_D r_T^2 N_v) \quad (7294)$$

$$\tau^3_{\gamma,\delta,w} = \sum_{i \in O} {}^2D^4_{i,w} Y^2_{i,\gamma} Y^{4,*}_{i,\delta} (3r_D r_T^2 N_o) \quad (7295)$$

$$\tau^4_{\gamma,\alpha} = \sum_{a \in V} W^4_{a,\alpha} Y^3_{a,\gamma} (2r_T r_V N_v) \quad (7296)$$

$$\tau^5_{\gamma,\alpha} = \sum_{i \in O} W^3_{i,\alpha} Y^4_{i,\gamma} (2r_T r_V N_o) \quad (7297)$$

$$\tau^6_{\gamma,\alpha} = \sum_{\beta \in B} X_{\alpha,\beta} \tau^4_{\gamma,\beta} \tau^5_{\gamma,\beta} (3r_T r_V^2) \quad (7298)$$

$$\tau^7_{\gamma,\alpha} = \sum_{a \in V} W^2_{a,\alpha} Y^3_{a,\gamma} (2r_T r_V N_v) \quad (7299)$$

$$\tau^8_{\gamma,\alpha} = \sum_{i \in O} W^1_{i,\alpha} Y^4_{i,\gamma} (2r_T r_V N_o) \quad (7300)$$

$$\tau^9_{\gamma,\delta} = \sum_{\alpha \in B} \tau^6_{\delta,\alpha} \tau^7_{\gamma,\alpha} \tau^8_{\gamma,\alpha} (3r_T^2 r_V) \quad (7301)$$

$$\tau^{10}_{\gamma,\delta} = \sum_{\epsilon \in A} Z_{\gamma,\epsilon} \tau^9_{\delta,\epsilon} (2r_T^3) \quad (7302)$$

$$\tau^{11}_{\gamma,\delta} = \sum_{\epsilon \in A} Z_{\gamma,\epsilon} \tau^{10}_{\delta,\epsilon} (2r_T^3) \quad (7303)$$

$$\tau_{\gamma,\delta,w}^{12} = \sum_{\epsilon \in A} \tau_{\gamma,\epsilon}^{11} \tau_{\epsilon,\delta,w}^2 \tau_{\epsilon,\delta,w}^3 \quad (3r_D r_T^3) \quad (7304)$$

$${}^2R_{\gamma,\delta}^z \leftarrow \sum_{\epsilon \in A} \sum_{w \in D} \tau_{\epsilon,\gamma,w}^0 \tau_{\epsilon,\gamma,w}^1 \tau_{\epsilon,\delta,w}^{12} \quad (3r_D r_T^3) \quad (7305)$$

Raw expression

$${}^2R_{\epsilon,\zeta}^z \leftarrow \sum_{i \in O} \sum_{j \in O} \sum_{k \in O} \sum_{l \in O} \sum_{a \in V} \sum_{b \in V} \sum_{c \in V} \sum_{d \in V} Y_{a,\epsilon}^{1,*} Y_{i,\epsilon}^{2,*} Y_{b,\zeta}^{3,*} Y_{j,\zeta}^{4,*} {}^2D_{a,i,b,j} {}^2T_{a,i,c,l} {}^2T_{d,k,b,j} V_{l,c,k,d} \quad (7306)$$

Factorized expression

$$\tau_{\gamma,\delta,w}^0 = \sum_{a \in V} {}^2D_{a,w}^1 Y_{a,\gamma}^1 Y_{a,\delta}^{1,*} \quad (3r_D r_T^2 N_v) \quad (7307)$$

$$\tau_{\gamma,\delta,w}^1 = \sum_{i \in O} {}^2D_{i,w}^2 Y_{i,\gamma}^2 Y_{i,\delta}^{2,*} \quad (3r_D r_T^2 N_o) \quad (7308)$$

$$\tau_{\gamma,\delta,w}^2 = \sum_{a \in V} {}^2D_{a,w}^3 Y_{a,\gamma}^3 Y_{a,\delta}^{3,*} \quad (3r_D r_T^2 N_v) \quad (7309)$$

$$\tau_{\gamma,\delta,w}^3 = \sum_{i \in O} {}^2D_{i,w}^4 Y_{i,\gamma}^4 Y_{i,\delta}^{4,*} \quad (3r_D r_T^2 N_o) \quad (7310)$$

$$\tau_{\gamma,\alpha}^4 = \sum_{a \in V} W_{a,\alpha}^2 Y_{a,\gamma}^3 \quad (2r_T r_V N_v) \quad (7311)$$

$$\tau_{\gamma,\alpha}^5 = \sum_{i \in O} W_{i,\alpha}^1 Y_{i,\gamma}^4 \quad (2r_T r_V N_o) \quad (7312)$$

$$\tau_{\gamma,\alpha}^6 = \sum_{a \in V} W_{a,\alpha}^4 Y_{a,\gamma}^1 \quad (2r_T r_V N_v) \quad (7313)$$

$$\tau_{\gamma,\alpha}^7 = \sum_{i \in O} W_{i,\alpha}^3 Y_{i,\gamma}^2 \quad (2r_T r_V N_o) \quad (7314)$$

$$\tau_{\gamma,\alpha}^8 = \sum_{\beta \in B} X_{\alpha,\beta} \tau_{\gamma,\beta}^6 \tau_{\gamma,\beta}^7 \quad (3r_T r_V^2) \quad (7315)$$

$$\tau_{\gamma,\delta}^9 = \sum_{\alpha \in B} \tau_{\delta,\alpha}^4 \tau_{\delta,\alpha}^5 \tau_{\gamma,\alpha}^8 \quad (3r_T^2 r_V) \quad (7316)$$

$$\tau_{\gamma,\delta}^{10} = \sum_{\epsilon \in A} Z_{\delta,\epsilon} \tau_{\gamma,\epsilon}^9 \quad (2r_T^3) \quad (7317)$$

$$\tau_{\gamma,\delta}^{11} = \sum_{\epsilon \in A} Z_{\epsilon,\delta} \tau_{\epsilon,\gamma}^{10} \quad (2r_T^3) \quad (7318)$$

$$\tau_{\gamma,\delta,w}^{12} = \sum_{\epsilon \in A} \tau_{\gamma,\epsilon}^{11} \tau_{\epsilon,\delta,w}^2 \tau_{\epsilon,\delta,w}^3 \quad (3r_D r_T^3) \quad (7319)$$

$${}^2R_{\gamma,\delta}^z \leftarrow \sum_{\epsilon \in A} \sum_{w \in D} \tau_{\epsilon,\gamma,w}^0 \tau_{\epsilon,\gamma,w}^1 \tau_{\epsilon,\delta,w}^{12} \quad (3r_D r_T^3) \quad (7320)$$

Raw expression

$${}^2R_{\epsilon,\zeta}^z \leftarrow \sum_{i \in O} \sum_{j \in O} \sum_{k \in O} \sum_{l \in O} \sum_{a \in V} \sum_{b \in V} \sum_{c \in V} \sum_{d \in V} Y_{a,\epsilon}^{1,*} Y_{i,\epsilon}^{2,*} Y_{b,\zeta}^{3,*} Y_{j,\zeta}^{4,*} {}^2D_{a,i,b,j} {}^2T_{b,j,c,l} {}^2T_{d,k,a,i} V_{k,d,l,c} \quad (7321)$$

Factorized expression

$$\tau_{\gamma,\alpha}^0 = \sum_{a \in V} W_{a,\alpha}^4 Y_{a,\gamma}^3 \quad (2r_T r_V N_v) \quad (7322)$$

$$\tau_{\gamma,\alpha}^1 = \sum_{i \in O} W_{i,\alpha}^3 Y_{i,\gamma}^4 \quad (2r_T r_V N_o) \quad (7323)$$

$$\tau_{\gamma,\alpha}^2 = \sum_{\beta \in B} X_{\alpha,\beta} \tau_{\gamma,\beta}^0 \tau_{\gamma,\beta}^1 \quad (3r_T r_V^2) \quad (7324)$$

$$\tau_{\gamma,\alpha}^3 = \sum_{a \in V} W_{a,\alpha}^2 Y_{a,\gamma}^1 \quad (2r_T r_V N_v) \quad (7325)$$

$$\tau_{\gamma,\alpha}^4 = \sum_{i \in O} W_{i,\alpha}^1 Y_{i,\gamma}^2 \quad (2r_T r_V N_o) \quad (7326)$$

$$\tau_{\gamma,\delta}^5 = \sum_{\alpha \in B} \tau_{\delta,\alpha}^2 \tau_{\gamma,\alpha}^3 \tau_{\gamma,\alpha}^4 \quad (3r_T^2 r_V) \quad (7327)$$

$$\tau_{\gamma,\delta}^6 = \sum_{\epsilon \in A} Z_{\delta,\epsilon} \tau_{\gamma,\epsilon}^5 \quad (2r_T^3) \quad (7328)$$

$$\tau_{\gamma,\delta}^7 = \sum_{\epsilon \in A} Z_{\epsilon,\delta} \tau_{\epsilon,\gamma}^6 \quad (2r_T^3) \quad (7329)$$



$$\tau^8_{\gamma,\delta,w} = \sum_{a \in V} {}^2D^1_{a,w} Y^3_{a,\gamma} Y^{1,*}_{a,\delta} \quad (3r_D r_T^2 N_v) \quad (7330)$$

$$\tau^6_{\gamma,\alpha} = \sum_{\beta \in B} X_{\alpha,\beta} \tau^4_{\gamma,\beta} \tau^5_{\gamma,\beta} \quad (3r_T r_V^2) \quad (7343)$$

$$\tau^9_{\gamma,\delta,w} = \sum_{i \in O} {}^2D^2_{i,w} Y^4_{i,\gamma} Y^{2,*}_{i,\delta} \quad (3r_D r_T^2 N_o) \quad (7331)$$

$$\tau^7_{\gamma,\alpha} = \sum_{a \in V} W^2_{a,\alpha} Y^1_{a,\gamma} \quad (2r_T r_V N_v) \quad (7344)$$

$$\tau^{10}_{\gamma,\delta,w} = \sum_{\epsilon \in A} \tau^7_{\gamma,\epsilon} \tau^8_{\epsilon,\delta,w} \tau^9_{\epsilon,\delta,w} \quad (3r_D r_T^3) \quad (7332)$$

$$\tau^8_{\gamma,\alpha} = \sum_{i \in O} W^1_{i,\alpha} Y^2_{i,\gamma} \quad (2r_T r_V N_o) \quad (7345)$$

$$\tau^{11}_{\gamma,\delta,w} = \sum_{a \in V} {}^2D^3_{a,w} Y^1_{a,\gamma} Y^{3,*}_{a,\delta} \quad (3r_D r_T^2 N_v) \quad (7333)$$

$$\tau^9_{\gamma,\delta} = \sum_{\alpha \in B} \tau^6_{\delta,\alpha} \tau^7_{\gamma,\alpha} \tau^8_{\gamma,\alpha} \quad (3r_T^2 r_V) \quad (7346)$$

$$\tau^{12}_{\gamma,\delta,w} = \sum_{i \in O} {}^2D^4_{i,w} Y^2_{i,\gamma} Y^{4,*}_{i,\delta} \quad (3r_D r_T^2 N_o) \quad (7334)$$

$$\tau^{10}_{\gamma,\delta} = \sum_{\epsilon \in A} Z_{\epsilon,\delta} \tau^9_{\gamma,\epsilon} \quad (2r_T^3) \quad (7347)$$

$${}^2R^z_{\gamma,\delta} \leftarrow \sum_{\epsilon \in A} \sum_{w \in D} \tau^{10}_{\epsilon,\gamma,w} \tau^{11}_{\epsilon,\delta,w} \tau^{12}_{\epsilon,\delta,w} \quad (3r_D r_T^3) \quad (7335)$$

$$\tau^{11}_{\gamma,\delta} = \sum_{\epsilon \in A} Z_{\epsilon,\gamma} \tau^{10}_{\epsilon,\delta} \quad (2r_T^3) \quad (7348)$$

Raw expression

$$\tau^{12}_{\gamma,\delta,w} = \sum_{\epsilon \in A} \tau^{11}_{\gamma,\epsilon} \tau^2_{\epsilon,\delta,w} \tau^3_{\epsilon,\delta,w} \quad (3r_D r_T^3) \quad (7349)$$

$${}^2R^z_{\epsilon,\zeta} \leftarrow \sum_{i \in O} \sum_{j \in O} \sum_{k \in O} \sum_{l \in O} \sum_{a \in V} \sum_{b \in V} \sum_{c \in V} \sum_{d \in V} Y^{1,*}_{a,\epsilon} Y^{2,*}_{i,\epsilon} Y^{3,*}_{b,\zeta} Y^{4,*}_{j,\zeta} {}^2D^{a,i,b,j} {}^2T_{c,k,a,i} {}^2T_{d,l,b,j} V_{k,c,l,d} \quad (7336)$$

$${}^2R^z_{\gamma,\delta} \leftarrow \sum_{\epsilon \in A} \sum_{w \in D} \tau^0_{\epsilon,\gamma,w} \tau^1_{\epsilon,\gamma,w} \tau^{12}_{\epsilon,\delta,w} \quad (3r_D r_T^3) \quad (7350)$$

Factorized expression

Raw expression

$$\tau^0_{\gamma,\delta,w} = \sum_{a \in V} {}^2D^1_{a,w} Y^3_{a,\gamma} Y^{1,*}_{a,\delta} \quad (3r_D r_T^2 N_v) \quad (7337)$$

$${}^2R^z_{\epsilon,\zeta} \leftarrow - \sum_{i \in O} \sum_{j \in O} \sum_{k \in O} \sum_{l \in O} \sum_{a \in V} \sum_{b \in V} \sum_{c \in V} \sum_{d \in V} \frac{1}{2} Y^{1,*}_{a,\epsilon} Y^{2,*}_{i,\epsilon} Y^{3,*}_{b,\zeta} Y^{4,*}_{j,\zeta} {}^2D^{a,i,b,j} {}^2T_{a,i,b,k} {}^2T_{c,j,d,l} V_{k,c,l,d} \quad (7351)$$

$$\tau^1_{\gamma,\delta,w} = \sum_{i \in O} {}^2D^2_{i,w} Y^4_{i,\gamma} Y^{2,*}_{i,\delta} \quad (3r_D r_T^2 N_o) \quad (7338)$$

Factorized expression

$$\tau^2_{\gamma,\delta,w} = \sum_{a \in V} {}^2D^3_{a,w} Y^3_{a,\gamma} Y^{3,*}_{a,\delta} \quad (3r_D r_T^2 N_v) \quad (7339)$$

$$\tau^0_{\gamma,\delta,w} = \sum_{a \in V} {}^2D^1_{a,w} Y^1_{a,\gamma} Y^{1,*}_{a,\delta} \quad (3r_D r_T^2 N_v) \quad (7352)$$

$$\tau^3_{\gamma,\delta,w} = \sum_{i \in O} {}^2D^4_{i,w} Y^4_{i,\gamma} Y^{4,*}_{i,\delta} \quad (3r_D r_T^2 N_o) \quad (7340)$$

$$\tau^1_{\gamma,\delta,w} = \sum_{i \in O} {}^2D^2_{i,w} Y^2_{i,\gamma} Y^{2,*}_{i,\delta} \quad (3r_D r_T^2 N_o) \quad (7353)$$

$$\tau^4_{\gamma,\alpha} = \sum_{a \in V} W^4_{a,\alpha} Y^1_{a,\gamma} \quad (2r_T r_V N_v) \quad (7341)$$

$$\tau^2_{\gamma,\delta,w} = \sum_{a \in V} {}^2D^3_{a,w} Y^1_{a,\gamma} Y^{3,*}_{a,\delta} \quad (3r_D r_T^2 N_v) \quad (7354)$$

$$\tau^5_{\gamma,\alpha} = \sum_{i \in O} W^3_{i,\alpha} Y^2_{i,\gamma} \quad (2r_T r_V N_o) \quad (7342)$$

$$\tau^3_{\gamma,\delta,w} = \sum_{i \in O} {}^2D^4_{i,w} Y^2_{i,\gamma} Y^{4,*}_{i,\delta} \quad (3r_D r_T^2 N_o) \quad (7355)$$

$$\tau^4_{\gamma,\alpha} = \sum_{a \in V} W^2_{a,\alpha} Y^3_{a,\gamma} \quad (2r_T r_V N_v) \quad (7356)$$

$$\tau^5_{\gamma,\alpha,i} = \sum_{\beta \in B} W^1_{i,\beta} X_{\beta,\alpha} \tau^4_{\gamma,\beta} \quad (3r_T r_V^2 N_o) \quad (7357)$$

$$\tau^6_{\gamma,\alpha} = \sum_{i \in O} W^3_{i,\alpha} Y^4_{i,\gamma} \quad (2r_T r_V N_o) \quad (7358)$$

$$\tau^7_{\gamma,\alpha} = \sum_{a \in V} W^4_{a,\alpha} Y^3_{a,\gamma} \quad (2r_T r_V N_v) \quad (7359)$$

$$\tau^8_{\gamma,\delta,i} = \sum_{\alpha \in B} \tau^6_{\gamma,\alpha} \tau^7_{\delta,\alpha} \tau^5_{\gamma,\alpha,i} \quad (3r_T^2 r_V N_o) \quad (7360)$$

$$\tau^9_{\gamma,\delta} = \sum_{i \in O} Y^4_{i,\delta} \tau^8_{\gamma,\delta,i} \quad (2r_T^2 N_o) \quad (7361)$$

$$\tau^{10}_{\gamma,\delta} = \sum_{\epsilon \in A} Z_{\gamma,\epsilon} \tau^9_{\delta,\epsilon} \quad (2r_T^3) \quad (7362)$$

$$\tau^{11}_{\gamma,\delta} = \sum_{\epsilon \in A} Z_{\gamma,\epsilon} \tau^{10}_{\delta,\epsilon} \quad (2r_T^3) \quad (7363)$$

$$\tau^{12}_{\gamma,\delta,w} = \sum_{\epsilon \in A} \tau^{11}_{\epsilon,\gamma} \tau^2_{\epsilon,\delta,w} \tau^3_{\epsilon,\delta,w} \quad (3r_D r_T^3) \quad (7364)$$

$${}^2R^z_{\gamma,\delta} \leftarrow - \sum_{\epsilon \in A} \sum_{w \in D} \frac{1}{2} \tau^0_{\epsilon,\gamma,w} \tau^1_{\epsilon,\gamma,w} \tau^{12}_{\epsilon,\delta,w} \quad (3r_D r_T^3) \quad (7365)$$

Raw expression

$${}^2R^z_{\epsilon,\zeta} \leftarrow - \sum_{i \in O} \sum_{j \in O} \sum_{k \in O} \sum_{l \in O} \sum_{a \in V} \sum_{b \in V} \sum_{c \in V} \sum_{d \in V} \frac{1}{2} Y^{1,*}_{a,\epsilon} Y^{2,*}_{i,\epsilon} Y^{3,*}_{b,\zeta} Y^{4,*}_{j,\zeta} {}^2D^{a,i,b,j} {}^2T_{a,i,b,l} {}^2T_{c,k,d,j} V_{l,d,k,c} \quad (7366)$$

Factorized expression

$$\tau^0_{\gamma,\delta,w} = \sum_{a \in V} {}^2D^1_{a,w} Y^1_{a,\gamma} Y^{1,*}_{a,\delta} \quad (3r_D r_T^2 N_v) \quad (7367)$$

$$\tau^1_{\gamma,\delta,w} = \sum_{i \in O} {}^2D^2_{i,w} Y^2_{i,\gamma} Y^{2,*}_{i,\delta} \quad (3r_D r_T^2 N_o) \quad (7368)$$

$$\tau^2_{\gamma,\alpha} = \sum_{i \in O} W^1_{i,\alpha} Y^2_{i,\gamma} \quad (2r_T r_V N_o) \quad (7369)$$

$$\tau^3_{\gamma,\alpha} = \sum_{a \in V} W^4_{a,\alpha} Y^3_{a,\gamma} \quad (2r_T r_V N_v) \quad (7370)$$

$$\tau^4_{\gamma,\alpha} = \sum_{i \in O} W^3_{i,\alpha} Y^4_{i,\gamma} \quad (2r_T r_V N_o) \quad (7371)$$

$$\tau^5_{\gamma,\alpha} = \sum_{\beta \in B} X_{\alpha,\beta} \tau^3_{\gamma,\beta} \tau^4_{\gamma,\beta} \quad (3r_T r_V^2) \quad (7372)$$

$$\tau^6_{\gamma,\alpha} = \sum_{\delta \in A} Z_{\gamma,\delta} \tau^5_{\delta,\alpha} \quad (2r_T^2 r_V) \quad (7373)$$

$$\tau^7_{\gamma,a} = \sum_{\alpha \in B} W^2_{a,\alpha} \tau^2_{\gamma,\alpha} \tau^6_{\gamma,\alpha} \quad (3r_T r_V N_v) \quad (7374)$$

$$\tau^8_{a,b} = \sum_{\gamma \in A} Y^1_{b,\gamma} \tau^7_{\gamma,a} \quad (2r_T N_v^2) \quad (7375)$$

$$\tau^9_{\gamma,a} = \sum_{b \in V} Y^3_{b,\gamma} \tau^8_{b,a} \quad (2r_T N_v^2) \quad (7376)$$

$$\tau^{10}_{\gamma,\delta,w} = \sum_{a \in V} {}^2D^3_{a,w} Y^{3,*}_{a,\delta} \tau^9_{\gamma,a} \quad (3r_D r_T^2 N_v) \quad (7377)$$

$$\tau^{11}_{\gamma,\delta,w} = \sum_{i \in O} {}^2D^4_{i,w} Y^4_{i,\gamma} Y^{4,*}_{i,\delta} \quad (3r_D r_T^2 N_o) \quad (7378)$$

$$\tau^{12}_{\gamma,\delta,w} = \sum_{\epsilon \in A} Z_{\gamma,\epsilon} \tau^{10}_{\epsilon,\delta,w} \tau^{11}_{\epsilon,\delta,w} \quad (3r_D r_T^3) \quad (7379)$$

$${}^2R^z_{\gamma,\delta} \leftarrow - \sum_{\epsilon \in A} \sum_{w \in D} \frac{1}{2} \tau^0_{\epsilon,\gamma,w} \tau^1_{\epsilon,\gamma,w} \tau^{12}_{\epsilon,\delta,w} \quad (3r_D r_T^3) \quad (7380)$$

Raw expression

$${}^2R^z_{\epsilon,\zeta} \leftarrow - \sum_{i \in O} \sum_{j \in O} \sum_{k \in O} \sum_{l \in O} \sum_{a \in V} \sum_{b \in V} \sum_{c \in V} \sum_{d \in V} \frac{1}{2} Y^{1,*}_{a,\epsilon} Y^{2,*}_{i,\epsilon} Y^{3,*}_{b,\zeta} Y^{4,*}_{j,\zeta} {}^2D^{a,i,b,j} {}^2T_{a,i,c,j} {}^2T_{b,k,d,l} V_{k,c,l,d} \quad (7381)$$

Factorized expression

$$\tau_{\gamma,\delta,w}^0 = \sum_{a \in V} {}^2D_{a,w}^1 Y_{a,\gamma}^1 Y_{a,\delta}^{1,*} \quad (3r_D r_T^2 N_v) \quad (7382)$$

$$\tau_{\gamma,\delta,w}^1 = \sum_{i \in O} {}^2D_{i,w}^2 Y_{i,\gamma}^2 Y_{i,\delta}^{2,*} \quad (3r_D r_T^2 N_o) \quad (7383)$$

$$\tau_{\gamma,\delta,w}^2 = \sum_{a \in V} {}^2D_{a,w}^3 Y_{a,\gamma}^1 Y_{a,\delta}^{3,*} \quad (3r_D r_T^2 N_v) \quad (7384)$$

$$\tau_{\gamma,\alpha}^3 = \sum_{a \in V} W_{a,\alpha}^2 Y_{a,\gamma}^3 \quad (2r_T r_V N_v) \quad (7385)$$

$$\tau_{\gamma,\alpha}^4 = \sum_{i \in O} W_{i,\alpha}^1 Y_{i,\gamma}^4 \quad (2r_T r_V N_o) \quad (7386)$$

$$\tau_{\gamma,\alpha}^5 = \sum_{\beta \in B} X_{\beta,\alpha} \tau_{\gamma,\beta}^3 \tau_{\gamma,\beta}^4 \quad (3r_T r_V^2) \quad (7387)$$

$$\tau_{\gamma,\alpha}^6 = \sum_{\delta \in A} Z_{\gamma,\delta} \tau_{\delta,\alpha}^5 \quad (2r_T^2 r_V) \quad (7388)$$

$$\tau_{\gamma,\alpha}^7 = \sum_{a \in V} W_{a,\alpha}^4 Y_{a,\gamma}^3 \quad (2r_T r_V N_v) \quad (7389)$$

$$\tau_{\gamma,\delta,i}^8 = \sum_{\alpha \in B} W_{i,\alpha}^3 \tau_{\gamma,\alpha}^6 \tau_{\delta,\alpha}^7 \quad (3r_T^2 r_V N_o) \quad (7390)$$

$$\tau_{\gamma,\delta,\epsilon}^9 = \sum_{i \in O} Y_{i,\gamma}^2 \tau_{\delta,\epsilon,i}^8 \quad (2r_T^3 N_o) \quad (7391)$$

$$\tau_{\gamma,\delta,i}^{10} = \sum_{\epsilon \in A} Z_{\gamma,\epsilon} Y_{i,\epsilon}^4 \tau_{\gamma,\delta,\epsilon}^9 \quad (3r_T^3 N_o) \quad (7392)$$

$$\tau_{\gamma,\delta,w}^{11} = \sum_{\epsilon \in A} \sum_{i \in O} {}^2D_{i,w}^4 Y_{i,\delta}^{4,*} \tau_{\epsilon,\gamma,i}^{10} \tau_{\epsilon,\delta,w}^2 \quad (4r_D r_T^3 N_o) \quad (7393)$$

$${}^2R_{\gamma,\delta}^z \leftarrow - \sum_{\epsilon \in A} \sum_{w \in D} \frac{1}{2} \tau_{\epsilon,\gamma,w}^0 \tau_{\epsilon,\gamma,w}^1 \tau_{\epsilon,\delta,w}^{11} \quad (3r_D r_T^3) \quad (7394)$$

Raw expression

$${}^2R_{\epsilon,\zeta}^z \leftarrow - \sum_{i \in O} \sum_{j \in O} \sum_{k \in O} \sum_{l \in O} \sum_{a \in V} \sum_{b \in V} \sum_{c \in V} \sum_{d \in V} \frac{1}{2} \quad (7395)$$

$$Y_{a,\epsilon}^{1,*} Y_{i,\epsilon}^{2,*} Y_{b,\zeta}^{3,*} Y_{j,\zeta}^{4,*}$$

$${}^2D_{a,i,b,j} {}^2T_{a,i,c,j} {}^2T_{d,k,b,l} V_{k,d,l,c}$$

Factorized expression

$$\tau_{\gamma,\delta,w}^0 = \sum_{a \in V} {}^2D_{a,w}^1 Y_{a,\gamma}^1 Y_{a,\delta}^{1,*} \quad (3r_D r_T^2 N_v) \quad (7396)$$

$$\tau_{\gamma,\delta,w}^1 = \sum_{i \in O} {}^2D_{i,w}^2 Y_{i,\gamma}^2 Y_{i,\delta}^{2,*} \quad (3r_D r_T^2 N_o) \quad (7397)$$

$$\tau_{\gamma,\delta,w}^2 = \sum_{a \in V} {}^2D_{a,w}^3 Y_{a,\gamma}^3 Y_{a,\delta}^{3,*} \quad (3r_D r_T^2 N_v) \quad (7398)$$

$$\tau_{\gamma,\alpha}^3 = \sum_{a \in V} W_{a,\alpha}^2 Y_{a,\gamma}^1 \quad (2r_T r_V N_v) \quad (7399)$$

$$\tau_{\gamma,\alpha}^4 = \sum_{a \in V} W_{a,\alpha}^4 Y_{a,\gamma}^3 \quad (2r_T r_V N_v) \quad (7400)$$

$$\tau_{\gamma,\alpha}^5 = \sum_{i \in O} W_{i,\alpha}^3 Y_{i,\gamma}^4 \quad (2r_T r_V N_o) \quad (7401)$$

$$\tau_{\gamma,\alpha}^6 = \sum_{\beta \in B} X_{\alpha,\beta} \tau_{\gamma,\beta}^4 \tau_{\gamma,\beta}^5 \quad (3r_T r_V^2) \quad (7402)$$

$$\tau_{\gamma,\alpha}^7 = \sum_{\delta \in A} Z_{\gamma,\delta} \tau_{\delta,\alpha}^6 \quad (2r_T^2 r_V) \quad (7403)$$

$$\tau_{\gamma,i}^8 = \sum_{\alpha \in B} W_{i,\alpha}^1 \tau_{\gamma,\alpha}^3 \tau_{\gamma,\alpha}^7 \quad (3r_T r_V N_o) \quad (7404)$$

$$\tau_{i,j}^9 = \sum_{\gamma \in A} Y_{j,\gamma}^2 \tau_{\gamma,i}^8 \quad (2r_T N_o^2) \quad (7405)$$

$$\tau_{\gamma,i}^{10} = \sum_{j \in O} Y_{j,\gamma}^4 \tau_{j,i}^9 \quad (2r_T N_o^2) \quad (7406)$$

$$\tau_{\gamma,\delta,w}^{11} = \sum_{i \in O} {}^2D_{i,w}^4 Y_{i,\delta}^{4,*} \tau_{\gamma,i}^{10} \quad (3r_D r_T^2 N_o) \quad (7407)$$

$$\tau_{\gamma,\delta,w}^{12} = \sum_{\epsilon \in A} Z_{\gamma,\epsilon} \tau_{\epsilon,\delta,w}^{11} \tau_{\epsilon,\delta,w}^2 \quad (3r_D r_T^3) \quad (7408)$$

$${}^2R_{\gamma,\delta}^z \leftarrow - \sum_{\epsilon \in A} \sum_{w \in D} \frac{1}{2} \tau_{\epsilon,\gamma,w}^0 \tau_{\epsilon,\gamma,w}^1 \tau_{\epsilon,\delta,w}^{12} \quad (3r_D r_T^3) \quad (7409)$$

Raw expression

$${}^2R^z_{\epsilon,\zeta} \leftarrow - \sum_{i \in O} \sum_{j \in O} \sum_{k \in O} \sum_{l \in O} \sum_{a \in V} \sum_{b \in V} \sum_{c \in V} \sum_{d \in V} \frac{1}{2} \quad (7410)$$

$$\begin{array}{c} Y^{1,*}_{a,\epsilon} \ Y^{2,*}_{i,\epsilon} \ Y^{3,*}_{b,\zeta} \ Y^{4,*}_{j,\zeta} \\ {}^2D^{a,i,b,j} \ {}^2T_{a,i,c,k} \ {}^2T_{b,j,d,l} \ V_{k,d,l,c} \end{array}$$

Factorized expression

$$\tau^0_{\gamma,\delta,w} = \sum_{a \in V} {}^2D^1_{a,w} Y^1_{a,\gamma} Y^{1,*}_{a,\delta} \quad (3r_D r_T^2 N_v) \quad (7411)$$

$$\tau^1_{\gamma,\delta,w} = \sum_{i \in O} {}^2D^2_{i,w} Y^2_{i,\gamma} Y^{2,*}_{i,\delta} \quad (3r_D r_T^2 N_o) \quad (7412)$$

$$\tau^2_{\gamma,\alpha} = \sum_{a \in V} W^2_{a,\alpha} Y^1_{a,\gamma} \quad (2r_T r_V N_v) \quad (7413)$$

$$\tau^3_{\gamma,\alpha} = \sum_{i \in O} W^1_{i,\alpha} Y^2_{i,\gamma} \quad (2r_T r_V N_o) \quad (7414)$$

$$\tau^4_{\gamma,\alpha} = \sum_{\beta \in B} X_{\beta,\alpha} \tau^2_{\gamma,\beta} \tau^3_{\gamma,\beta} \quad (3r_T r_V^2) \quad (7415)$$

$$\tau^5_{\gamma,\alpha} = \sum_{\delta \in A} Z_{\delta,\gamma} \tau^4_{\delta,\alpha} \quad (2r_T^2 r_V) \quad (7416)$$

$$\tau^6_{\gamma,\alpha} = \sum_{i \in O} W^3_{i,\alpha} Y^4_{i,\gamma} \quad (2r_T r_V N_o) \quad (7417)$$

$$\tau^7_{\gamma,a} = \sum_{\alpha \in B} W^4_{a,\alpha} \tau^5_{\gamma,\alpha} \tau^6_{\gamma,\alpha} \quad (3r_T r_V N_v) \quad (7418)$$

$$\tau^8_{\gamma,\delta} = \sum_{a \in V} Y^3_{a,\delta} \tau^7_{\gamma,a} \quad (2r_T^2 N_v) \quad (7419)$$

$$\tau^9_{\gamma,a} = \sum_{\delta \in A} Y^3_{a,\delta} \tau^8_{\delta,\gamma} \quad (2r_T^2 N_v) \quad (7420)$$

$$\tau^{10}_{\gamma,\delta,w} = \sum_{a \in V} {}^2D^3_{a,w} Y^{3,*}_{a,\delta} \tau^9_{\gamma,a} \quad (3r_D r_T^2 N_v) \quad (7421)$$

$$\tau^{11}_{\gamma,\delta,w} = \sum_{i \in O} {}^2D^4_{i,w} Y^4_{i,\gamma} Y^{4,*}_{i,\delta} \quad (3r_D r_T^2 N_o) \quad (7422)$$

$$\tau^{12}_{\gamma,\delta,w} = \sum_{\epsilon \in A} Z_{\gamma,\epsilon} \tau^{10}_{\epsilon,\delta,w} \tau^{11}_{\epsilon,\delta,w} \quad (3r_D r_T^3) \quad (7423)$$

$${}^2R^z_{\gamma,\delta} \leftarrow - \sum_{\epsilon \in A} \sum_{w \in D} \frac{1}{2} \tau^0_{\epsilon,\gamma,w} \tau^1_{\epsilon,\gamma,w} \tau^{12}_{\epsilon,\delta,w} \quad (3r_D r_T^3) \quad (7424)$$

Raw expression

$${}^2R^z_{\epsilon,\zeta} \leftarrow - \sum_{i \in O} \sum_{j \in O} \sum_{k \in O} \sum_{l \in O} \sum_{a \in V} \sum_{b \in V} \sum_{c \in V} \sum_{d \in V} \frac{1}{2} \quad (7425)$$

$$\begin{array}{c} Y^{1,*}_{a,\epsilon} \ Y^{2,*}_{i,\epsilon} \ Y^{3,*}_{b,\zeta} \ Y^{4,*}_{j,\zeta} \\ {}^2D^{a,i,b,j} \ {}^2T_{a,i,c,k} \ {}^2T_{d,j,b,l} \ V_{k,c,l,d} \end{array}$$

Factorized expression

$$\tau^0_{\gamma,\delta,w} = \sum_{a \in V} {}^2D^1_{a,w} Y^1_{a,\gamma} Y^{1,*}_{a,\delta} \quad (3r_D r_T^2 N_v) \quad (7426)$$

$$\tau^1_{\gamma,\delta,w} = \sum_{i \in O} {}^2D^2_{i,w} Y^2_{i,\gamma} Y^{2,*}_{i,\delta} \quad (3r_D r_T^2 N_o) \quad (7427)$$

$$\tau^2_{\gamma,\delta,w} = \sum_{a \in V} {}^2D^3_{a,w} Y^3_{a,\gamma} Y^{3,*}_{a,\delta} \quad (3r_D r_T^2 N_v) \quad (7428)$$

$$\tau^3_{\gamma,\delta,w} = \sum_{i \in O} {}^2D^4_{i,w} Y^4_{i,\gamma} Y^{4,*}_{i,\delta} \quad (3r_D r_T^2 N_o) \quad (7429)$$

$$\tau^4_{\gamma,\alpha} = \sum_{a \in V} W^2_{a,\alpha} Y^1_{a,\gamma} \quad (2r_T r_V N_v) \quad (7430)$$

$$\tau^5_{\gamma,\alpha,i} = \sum_{\beta \in B} W^1_{i,\beta} X_{\beta,\alpha} \tau^4_{\gamma,\beta} \quad (3r_T r_V^2 N_o) \quad (7431)$$

$$\tau^6_{\gamma,\alpha} = \sum_{i \in O} W^3_{i,\alpha} Y^2_{i,\gamma} \quad (2r_T r_V N_o) \quad (7432)$$

$$\tau^7_{\gamma,\alpha} = \sum_{a \in V} W^4_{a,\alpha} Y^3_{a,\gamma} \quad (2r_T r_V N_v) \quad (7433)$$

$$\tau^8_{\gamma,\delta,i} = \sum_{\alpha \in B} \tau^6_{\gamma,\alpha} \tau^7_{\delta,\alpha} \tau^5_{\gamma,\alpha,i} \quad (3r_T^2 r_V N_o) \quad (7434)$$

$$\tau^9_{\gamma,\delta} = \sum_{i \in O} Y^4_{i,\delta} \tau^8_{\gamma,\delta,i} \quad (2r_T^2 N_o) \quad (7435)$$

$$\tau^{10}_{\gamma,\delta} = \sum_{\epsilon \in A} Z_{\delta,\epsilon} \tau^9_{\gamma,\epsilon} \quad (2r_T^3) \quad (7436)$$

$$\tau^{11}_{\gamma,\delta} = \sum_{\epsilon \in A} Z_{\epsilon,\delta} \tau^{10}_{\epsilon,\gamma} \quad (2r_T^3) \quad (7437)$$

$$\tau^9_{\gamma,\delta,\epsilon} = \sum_{i \in O} Z_{\gamma,\epsilon} Y^4_{i,\epsilon} \tau^8_{\gamma,\delta,i} \quad (3r_T^3 N_o) \quad (7450)$$

$$\tau^{12}_{\gamma,\delta,w} = \sum_{\epsilon \in A} \tau^{11}_{\gamma,\epsilon} \tau^2_{\epsilon,\delta,w} \tau^3_{\epsilon,\delta,w} \quad (3r_D r_T^3) \quad (7438)$$

$$\tau^{10}_{\gamma,\delta,i} = \sum_{\epsilon \in A} Y^2_{i,\epsilon} \tau^9_{\epsilon,\gamma,\delta} \quad (2r_T^3 N_o) \quad (7451)$$

$${}^2R^z_{\gamma,\delta} \leftarrow - \sum_{\epsilon \in A} \sum_{w \in D} \frac{1}{2} \tau^0_{\epsilon,\gamma,w} \tau^1_{\epsilon,\gamma,w} \tau^{12}_{\epsilon,\delta,w} \quad (3r_D r_T^3) \quad (7439)$$

$$\tau^{11}_{\gamma,\delta,w} = \sum_{\epsilon \in A} \sum_{i \in O} {}^2D^4_{i,w} Y^{4,*}_{i,\delta} \tau^{10}_{\gamma,\epsilon,i} \tau^2_{\epsilon,\delta,w} \quad (4r_D r_T^3 N_o) \quad (7452)$$

Raw expression

$${}^2R^z_{\epsilon,\zeta} \leftarrow - \sum_{i \in O} \sum_{j \in O} \sum_{k \in O} \sum_{l \in O} \sum_{a \in V} \sum_{b \in V} \sum_{c \in V} \sum_{d \in V} \frac{1}{2} \quad (7440)$$

$$Y^{1,*}_{a,\epsilon} Y^{2,*}_{i,\epsilon} Y^{3,*}_{b,\zeta} Y^{4,*}_{j,\zeta}$$

$${}^2D^{a,i,b,j}_{a,i,c,l} {}^2T_{b,k,d,j} V_{l,c,k,d}$$

$${}^2R^z_{\gamma,\delta} \leftarrow - \sum_{\epsilon \in A} \sum_{w \in D} \frac{1}{2} \tau^0_{\epsilon,\gamma,w} \tau^1_{\epsilon,\gamma,w} \tau^{11}_{\epsilon,\delta,w} \quad (3r_D r_T^3) \quad (7453)$$

Raw expression

$${}^2R^z_{\epsilon,\zeta} \leftarrow - \sum_{i \in O} \sum_{j \in O} \sum_{k \in O} \sum_{l \in O} \sum_{a \in V} \sum_{b \in V} \sum_{c \in V} \sum_{d \in V} \frac{1}{2} \quad (7454)$$

$$Y^{1,*}_{a,\epsilon} Y^{2,*}_{i,\epsilon} Y^{3,*}_{b,\zeta} Y^{4,*}_{j,\zeta}$$

$${}^2D^{a,i,b,j}_{a,i,c,l} {}^2T_{d,k,b,j} V_{l,d,k,c}$$

Factorized expression

$$\tau^0_{\gamma,\delta,w} = \sum_{a \in V} {}^2D^1_{a,w} Y^1_{a,\gamma} Y^{1,*}_{a,\delta} \quad (3r_D r_T^2 N_v) \quad (7441)$$

Factorized expression

$$\tau^0_{\gamma,\delta,w} = \sum_{a \in V} {}^2D^3_{a,w} Y^3_{a,\gamma} Y^{3,*}_{a,\delta} \quad (3r_D r_T^2 N_v) \quad (7455)$$

$$\tau^2_{\gamma,\delta,w} = \sum_{a \in V} {}^2D^3_{a,w} Y^3_{a,\gamma} Y^{3,*}_{a,\delta} \quad (3r_D r_T^2 N_v) \quad (7443)$$

$$\tau^1_{\gamma,\alpha} = \sum_{a \in V} W^4_{a,\alpha} Y^1_{a,\gamma} \quad (2r_T r_V N_v) \quad (7456)$$

$$\tau^3_{\gamma,\alpha} = \sum_{a \in V} W^4_{a,\alpha} Y^1_{a,\gamma} \quad (2r_T r_V N_v) \quad (7444)$$

$$\tau^2_{\gamma,\alpha} = \sum_{i \in O} W^3_{i,\alpha} Y^2_{i,\gamma} \quad (2r_T r_V N_o) \quad (7457)$$

$$\tau^4_{\gamma,\alpha} = \sum_{a \in V} W^2_{a,\alpha} Y^3_{a,\gamma} \quad (2r_T r_V N_v) \quad (7445)$$

$$\tau^3_{\gamma,\alpha} = \sum_{\beta \in B} X_{\alpha,\beta} \tau^1_{\gamma,\beta} \tau^2_{\gamma,\beta} \quad (3r_T r_V^2) \quad (7458)$$

$$\tau^5_{\gamma,\alpha} = \sum_{i \in O} W^1_{i,\alpha} Y^4_{i,\gamma} \quad (2r_T r_V N_o) \quad (7446)$$

$$\tau^4_{\gamma,\alpha} = \sum_{\delta \in A} Z_{\delta,\gamma} \tau^3_{\delta,\alpha} \quad (2r_T^2 r_V) \quad (7459)$$

$$\tau^6_{\gamma,\alpha} = \sum_{\beta \in B} X_{\beta,\alpha} \tau^4_{\gamma,\beta} \tau^5_{\gamma,\beta} \quad (3r_T r_V^2) \quad (7447)$$

$$\tau^5_{\gamma,\alpha} = \sum_{a \in V} W^2_{a,\alpha} Y^3_{a,\gamma} \quad (2r_T r_V N_v) \quad (7460)$$

$$\tau^7_{\gamma,\alpha} = \sum_{\delta \in A} Z_{\gamma,\delta} \tau^6_{\delta,\alpha} \quad (2r_T^2 r_V) \quad (7448)$$

$$\tau^6_{\gamma,i} = \sum_{\alpha \in B} W^1_{i,\alpha} \tau^4_{\gamma,\alpha} \tau^5_{\gamma,\alpha} \quad (3r_T r_V N_o) \quad (7461)$$

$$\tau^8_{\gamma,\delta,i} = \sum_{\alpha \in B} W^3_{i,\alpha} \tau^3_{\gamma,\alpha} \tau^7_{\delta,\alpha} \quad (3r_T^2 r_V N_o) \quad (7449)$$

$$\tau^7_{i,j} = \sum_{\gamma \in A} Y^4_{j,\gamma} \tau^6_{\gamma,i} \quad (2r_T N_o^2) \quad (7462)$$

$$\tau^8_{\gamma,i} = \sum_{j \in O} Y^4_{j,\gamma} \tau^7_{j,i} \quad (2r_T N_o^2) \quad (7463)$$

$$\tau^6_{i,j} = \sum_{\gamma \in A} Y^4_{j,\gamma} \tau^5_{\gamma,i} \quad (2r_T N_o^2) \quad (7476)$$

$$\tau^9_{\gamma,\delta,w} = \sum_{i \in O} {}^2D^4_{i,w} Y^{4,*}_{i,\delta} \tau^8_{\gamma,i} \quad (3r_D r_T^2 N_o) \quad (7464)$$

$$\tau^7_{\gamma,i} = \sum_{j \in O} Y^2_{j,\gamma} \tau^6_{j,i} \quad (2r_T N_o^2) \quad (7477)$$

$$\tau^{10}_{\gamma,\delta,w} = \sum_{\epsilon \in A} Z_{\gamma,\epsilon} \tau^0_{\epsilon,\delta,w} \tau^9_{\epsilon,\delta,w} \quad (3r_D r_T^3) \quad (7465)$$

$$\tau^8_{\gamma,\delta,w} = \sum_{i \in O} {}^2D^2_{i,w} Y^{2,*}_{i,\delta} \tau^7_{\gamma,i} \quad (3r_D r_T^2 N_o) \quad (7478)$$

$$\tau^{11}_{\gamma,\delta,w} = \sum_{a \in V} {}^2D^1_{a,w} Y^1_{a,\gamma} Y^{1,*}_{a,\delta} \quad (3r_D r_T^2 N_v) \quad (7466)$$

$$\tau^9_{\gamma,\delta,w} = \sum_{a \in V} {}^2D^1_{a,w} Y^1_{a,\gamma} Y^{1,*}_{a,\delta} \quad (3r_D r_T^2 N_v) \quad (7479)$$

$$\tau^{12}_{\gamma,\delta,w} = \sum_{i \in O} {}^2D^2_{i,w} Y^2_{i,\gamma} Y^{2,*}_{i,\delta} \quad (3r_D r_T^2 N_o) \quad (7467)$$

$$\tau^{10}_{\gamma,\delta,w} = \sum_{a \in V} {}^2D^3_{a,w} Y^3_{a,\gamma} Y^{3,*}_{a,\delta} \quad (3r_D r_T^2 N_v) \quad (7480)$$

$${}^2R^z_{\gamma,\delta} \leftarrow - \sum_{\epsilon \in A} \sum_{w \in D} \frac{1}{2} \tau^{10}_{\epsilon,\delta,w} \tau^{11}_{\epsilon,\gamma,w} \tau^{12}_{\epsilon,\gamma,w} \quad (3r_D r_T^3) \quad (7468)$$

$$\tau^{11}_{\gamma,\delta,w} = \sum_{i \in O} {}^2D^4_{i,w} Y^4_{i,\gamma} Y^{4,*}_{i,\delta} \quad (3r_D r_T^2 N_o) \quad (7481)$$

Raw expression

$$\tau^{12}_{\gamma,\delta,w} = \sum_{\epsilon \in A} Z_{\gamma,\epsilon} \tau^{10}_{\epsilon,\delta,w} \tau^{11}_{\epsilon,\delta,w} \quad (3r_D r_T^3) \quad (7482)$$

$${}^2R^z_{\epsilon,\zeta} \leftarrow - \sum_{i \in O} \sum_{j \in O} \sum_{k \in O} \sum_{l \in O} \sum_{a \in V} \sum_{b \in V} \sum_{c \in V} \sum_{d \in V} \frac{1}{2} \quad (7469)$$

$$\begin{aligned} & Y^{1,*}_{a,\epsilon} Y^{2,*}_{i,\epsilon} Y^{3,*}_{b,\zeta} Y^{4,*}_{j,\zeta} \\ & {}^2D^{a,i,b,j} {}^2T_{a,k,b,j} {}^2T_{c,i,d,l} V_{k,c,l,d} \end{aligned}$$

$${}^2R^z_{\gamma,\delta} \leftarrow - \sum_{\epsilon \in A} \sum_{w \in D} \frac{1}{2} \tau^{12}_{\epsilon,\delta,w} \tau^8_{\epsilon,\gamma,w} \tau^9_{\epsilon,\gamma,w} \quad (3r_D r_T^3) \quad (7483)$$

Factorized expression

Raw expression

$$\tau^0_{\gamma,\alpha} = \sum_{a \in V} W^4_{a,\alpha} Y^1_{a,\gamma} \quad (2r_T r_V N_v) \quad (7470)$$

$${}^2R^z_{\epsilon,\zeta} \leftarrow - \sum_{i \in O} \sum_{j \in O} \sum_{k \in O} \sum_{l \in O} \sum_{a \in V} \sum_{b \in V} \sum_{c \in V} \sum_{d \in V} \frac{1}{2} \quad (7484)$$

$$\begin{aligned} & Y^{1,*}_{a,\epsilon} Y^{2,*}_{i,\epsilon} Y^{3,*}_{b,\zeta} Y^{4,*}_{j,\zeta} \\ & {}^2D^{a,i,b,j} {}^2T_{a,k,b,j} {}^2T_{c,l,d,i} V_{k,d,l,c} \end{aligned}$$

$$\tau^1_{\gamma,\alpha} = \sum_{i \in O} W^3_{i,\alpha} Y^2_{i,\gamma} \quad (2r_T r_V N_o) \quad (7471)$$

Factorized expression

$$\tau^2_{\gamma,\alpha} = \sum_{\beta \in B} X_{\alpha,\beta} \tau^0_{\gamma,\beta} \tau^1_{\gamma,\beta} \quad (3r_T r_V^2) \quad (7472)$$

$$\tau^0_{\gamma,\delta,w} = \sum_{a \in V} {}^2D^1_{a,w} Y^1_{a,\gamma} Y^{1,*}_{a,\delta} \quad (3r_D r_T^2 N_v) \quad (7485)$$

$$\tau^3_{\gamma,\alpha} = \sum_{\delta \in A} Z_{\delta,\gamma} \tau^2_{\delta,\alpha} \quad (2r_T^2 r_V) \quad (7473)$$

$$\tau^1_{\gamma,\alpha} = \sum_{a \in V} W^2_{a,\alpha} Y^3_{a,\gamma} \quad (2r_T r_V N_v) \quad (7486)$$

$$\tau^4_{\gamma,\alpha} = \sum_{a \in V} W^2_{a,\alpha} Y^3_{a,\gamma} \quad (2r_T r_V N_v) \quad (7474)$$

$$\tau^2_{\gamma,\alpha} = \sum_{a \in V} W^4_{a,\alpha} Y^1_{a,\gamma} \quad (2r_T r_V N_v) \quad (7487)$$

$$\tau^5_{\gamma,i} = \sum_{\alpha \in B} W^1_{i,\alpha} \tau^3_{\gamma,\alpha} \tau^4_{\gamma,\alpha} \quad (3r_T r_V N_o) \quad (7475)$$

$$\tau^3_{\gamma,\alpha} = \sum_{i \in O} W^3_{i,\alpha} Y^2_{i,\gamma} \quad (2r_T r_V N_o) \quad (7488)$$

$$\tau^4_{\gamma,\alpha} = \sum_{\beta \in B} X_{\alpha,\beta} \tau^2_{\gamma,\beta} \tau^3_{\gamma,\beta} \quad (3r_T r_V^2) \quad (7489)$$

$$\tau^3_{\gamma,\alpha} = \sum_{\beta \in B} X_{\alpha,\beta} \tau^1_{\gamma,\beta} \tau^2_{\gamma,\beta} \quad (3r_T r_V^2) \quad (7502)$$

$$\tau^5_{\gamma,\alpha} = \sum_{\delta \in A} Z_{\delta,\gamma} \tau^4_{\delta,\alpha} \quad (2r_T^2 r_V) \quad (7490)$$

$$\tau^4_{\gamma,\alpha} = \sum_{\delta \in A} Z_{\gamma,\delta} \tau^3_{\delta,\alpha} \quad (2r_T^2 r_V) \quad (7503)$$

$$\tau^6_{\gamma,\delta,i} = \sum_{\alpha \in B} W^1_{i,\alpha} \tau^1_{\delta,\alpha} \tau^5_{\gamma,\alpha} \quad (3r_T^2 r_V N_o) \quad (7491)$$

$$\tau^5_{\gamma,a} = \sum_{\alpha \in B} W^2_{a,\alpha} \tau^0_{\gamma,\alpha} \tau^4_{\gamma,\alpha} \quad (3r_T r_V N_v) \quad (7504)$$

$$\tau^7_{\gamma,\delta,\epsilon} = \sum_{i \in O} Y^2_{i,\gamma} \tau^6_{\delta,\epsilon,i} \quad (2r_T^3 N_o) \quad (7492)$$

$$\tau^6_{a,b} = \sum_{\gamma \in A} Y^1_{b,\gamma} \tau^5_{\gamma,a} \quad (2r_T N_v^2) \quad (7505)$$

$$\tau^8_{\gamma,\delta,i} = \sum_{\epsilon \in A} Z_{\gamma,\epsilon} Y^4_{i,\epsilon} \tau^7_{\gamma,\delta,\epsilon} \quad (3r_T^3 N_o) \quad (7493)$$

$$\tau^7_{\gamma,a} = \sum_{b \in V} Y^3_{b,\gamma} \tau^6_{b,a} \quad (2r_T N_v^2) \quad (7506)$$

$$\tau^9_{\gamma,\delta,w} = \sum_{\epsilon \in A} \sum_{i \in O} {}^2D^2_{i,w} Y^{2,*}_{i,\delta} \tau^0_{\epsilon,\delta,w} \tau^8_{\epsilon,\gamma,i} \quad (4r_D r_T^3 N_o) \quad (7494)$$

$$\tau^8_{\gamma,\delta,w} = \sum_{a \in V} {}^2D^1_{a,w} Y^{1,*}_{a,\delta} \tau^7_{\gamma,a} \quad (3r_D r_T^2 N_v) \quad (7507)$$

$$\tau^{10}_{\gamma,\delta,w} = \sum_{a \in V} {}^2D^3_{a,w} Y^3_{a,\gamma} Y^{3,*}_{a,\delta} \quad (3r_D r_T^2 N_v) \quad (7495)$$

$$\tau^9_{\gamma,\delta,w} = \sum_{i \in O} {}^2D^2_{i,w} Y^4_{i,\gamma} Y^{2,*}_{i,\delta} \quad (3r_D r_T^2 N_o) \quad (7508)$$

$$\tau^{11}_{\gamma,\delta,w} = \sum_{i \in O} {}^2D^4_{i,w} Y^4_{i,\gamma} Y^{4,*}_{i,\delta} \quad (3r_D r_T^2 N_o) \quad (7496)$$

$$\tau^{10}_{\gamma,\delta,w} = \sum_{a \in V} {}^2D^3_{a,w} Y^1_{a,\gamma} Y^{3,*}_{a,\delta} \quad (3r_D r_T^2 N_v) \quad (7509)$$

$${}^2R^z_{\gamma,\delta} \leftarrow - \sum_{\epsilon \in A} \sum_{w \in D} \frac{1}{2} \tau^{10}_{\epsilon,\delta,w} \tau^{11}_{\epsilon,\delta,w} \tau^9_{\epsilon,\gamma,w} \quad (3r_D r_T^3) \quad (7497)$$

$$\tau^{11}_{\gamma,\delta,w} = \sum_{i \in O} {}^2D^4_{i,w} Y^2_{i,\gamma} Y^{4,*}_{i,\delta} \quad (3r_D r_T^2 N_o) \quad (7510)$$

Raw expression

$$\tau^{12}_{\gamma,\delta,w} = \sum_{\epsilon \in A} Z_{\epsilon,\gamma} \tau^{10}_{\epsilon,\delta,w} \tau^{11}_{\epsilon,\delta,w} \quad (3r_D r_T^3) \quad (7511)$$

$${}^2R^z_{\epsilon,\zeta} \leftarrow - \sum_{i \in O} \sum_{j \in O} \sum_{k \in O} \sum_{l \in O} \sum_{a \in V} \sum_{b \in V} \sum_{c \in V} \sum_{d \in V} \frac{1}{2} Y^{1,*}_{a,\epsilon} Y^{2,*}_{i,\epsilon} Y^{3,*}_{b,\zeta} Y^{4,*}_{j,\zeta} {}^2D^{a,i,b,j} {}^2T_{a,k,c,i} {}^2T_{d,l,b,j} V_{k,c,l,d} \quad (7498)$$

$${}^2R^z_{\gamma,\delta} \leftarrow - \sum_{\epsilon \in A} \sum_{w \in D} \frac{1}{2} \tau^{12}_{\epsilon,\delta,w} \tau^8_{\epsilon,\gamma,w} \tau^9_{\epsilon,\gamma,w} \quad (3r_D r_T^3) \quad (7512)$$

Factorized expression

Raw expression

$$\tau^0_{\gamma,\alpha} = \sum_{i \in O} W^1_{i,\alpha} Y^2_{i,\gamma} \quad (2r_T r_V N_o) \quad (7499)$$

$${}^2R^z_{\epsilon,\zeta} \leftarrow - \sum_{i \in O} \sum_{j \in O} \sum_{k \in O} \sum_{l \in O} \sum_{a \in V} \sum_{b \in V} \sum_{c \in V} \sum_{d \in V} \frac{1}{2} Y^{1,*}_{a,\epsilon} Y^{2,*}_{i,\epsilon} Y^{3,*}_{b,\zeta} Y^{4,*}_{j,\zeta} {}^2D^{a,i,b,j} {}^2T_{a,k,d,i} {}^2T_{b,j,c,l} V_{k,d,l,c} \quad (7513)$$

$$\tau^1_{\gamma,\alpha} = \sum_{a \in V} W^4_{a,\alpha} Y^3_{a,\gamma} \quad (2r_T r_V N_v) \quad (7500)$$

Factorized expression

$$\tau^2_{\gamma,\alpha} = \sum_{i \in O} W^3_{i,\alpha} Y^4_{i,\gamma} \quad (2r_T r_V N_o) \quad (7501)$$

$$\tau^0_{\gamma,\delta,w} = \sum_{a \in V} {}^2D^1_{a,w} Y^1_{a,\gamma} Y^{1,*}_{a,\delta} \quad (3r_D r_T^2 N_v) \quad (7514)$$

Factorized expression

$$\tau^1_{\gamma,\alpha} = \sum_{a \in V} W^4_{a,\alpha} Y^3_{a,\gamma} \quad (2r_T r_V N_v) \quad (7515)$$

$$\tau^2_{\gamma,\alpha} = \sum_{i \in O} W^3_{i,\alpha} Y^4_{i,\gamma} \quad (2r_T r_V N_o) \quad (7516)$$

$$\tau^3_{\gamma,\alpha} = \sum_{\beta \in B} X_{\alpha,\beta} \tau^1_{\gamma,\beta} \tau^2_{\gamma,\beta} \quad (3r_T r_V^2) \quad (7517)$$

$$\tau^4_{\gamma,\alpha} = \sum_{\delta \in A} Z_{\gamma,\delta} \tau^3_{\delta,\alpha} \quad (2r_T^2 r_V) \quad (7518)$$

$$\tau^5_{\gamma,\alpha} = \sum_{a \in V} W^2_{a,\alpha} Y^3_{a,\gamma} \quad (2r_T r_V N_v) \quad (7519)$$

$$\tau^6_{\gamma,\delta,i} = \sum_{\alpha \in B} W^1_{i,\alpha} \tau^4_{\gamma,\alpha} \tau^5_{\delta,\alpha} \quad (3r_T^2 r_V N_o) \quad (7520)$$

$$\tau^7_{\gamma,\delta,\epsilon} = \sum_{i \in O} Y^2_{i,\gamma} Z_{\gamma,\epsilon} \tau^6_{\delta,\epsilon,i} \quad (3r_T^3 N_o) \quad (7521)$$

$$\tau^8_{\gamma,\delta,i} = \sum_{\epsilon \in A} Y^4_{i,\epsilon} \tau^7_{\gamma,\delta,\epsilon} \quad (2r_T^3 N_o) \quad (7522)$$

$$\tau^9_{\gamma,\delta,w} = \sum_{\epsilon \in A} \sum_{i \in O} {}^2D^2_{i,w} Y^{2,*}_{i,\delta} \tau^0_{\epsilon,\delta,w} \tau^8_{\epsilon,\gamma,i} \quad (4r_D r_T^3 N_o) \quad (7523)$$

$$\tau^{10}_{\gamma,\delta,w} = \sum_{a \in V} {}^2D^3_{a,w} Y^1_{a,\gamma} Y^{3,*}_{a,\delta} \quad (3r_D r_T^2 N_v) \quad (7524)$$

$$\tau^{11}_{\gamma,\delta,w} = \sum_{i \in O} {}^2D^4_{i,w} Y^2_{i,\gamma} Y^{4,*}_{i,\delta} \quad (3r_D r_T^2 N_o) \quad (7525)$$

$${}^2R^z_{\gamma,\delta} \leftarrow - \sum_{\epsilon \in A} \sum_{w \in D} \frac{1}{2} \tau^{10}_{\epsilon,\delta,w} \tau^{11}_{\epsilon,\delta,w} \tau^9_{\epsilon,\gamma,w} \quad (3r_D r_T^3) \quad (7526)$$

Raw expression

$${}^2R^z_{\epsilon,\zeta} \leftarrow - \sum_{i \in O} \sum_{j \in O} \sum_{k \in O} \sum_{l \in O} \sum_{a \in V} \sum_{b \in V} \sum_{c \in V} \sum_{d \in V} \frac{1}{2} \quad (7527)$$

$$Y^{1,*}_{a,\epsilon} Y^{2,*}_{i,\epsilon} Y^{3,*}_{b,\zeta} Y^{4,*}_{j,\zeta}$$

$${}^2D^{a,i,b,j} {}^2T_{a,k,d,l} {}^2T_{b,j,c,i} V_{k,c,l,d}$$

$$\tau^0_{\gamma,\delta,w} = \sum_{i \in O} {}^2D^2_{i,w} Y^2_{i,\gamma} Y^{2,*}_{i,\delta} \quad (3r_D r_T^2 N_o) \quad (7528)$$

$$\tau^1_{\gamma,\alpha} = \sum_{i \in O} W^1_{i,\alpha} Y^2_{i,\gamma} \quad (2r_T r_V N_o) \quad (7529)$$

$$\tau^2_{\gamma,\alpha} = \sum_{a \in V} W^4_{a,\alpha} Y^3_{a,\gamma} \quad (2r_T r_V N_v) \quad (7530)$$

$$\tau^3_{\gamma,\alpha} = \sum_{i \in O} W^3_{i,\alpha} Y^4_{i,\gamma} \quad (2r_T r_V N_o) \quad (7531)$$

$$\tau^4_{\gamma,\alpha} = \sum_{\beta \in B} X_{\alpha,\beta} \tau^2_{\gamma,\beta} \tau^3_{\gamma,\beta} \quad (3r_T r_V^2) \quad (7532)$$

$$\tau^5_{\gamma,\alpha} = \sum_{\delta \in A} Z_{\gamma,\delta} \tau^4_{\delta,\alpha} \quad (2r_T^2 r_V) \quad (7533)$$

$$\tau^6_{\gamma,a} = \sum_{\alpha \in B} W^2_{a,\alpha} \tau^1_{\gamma,\alpha} \tau^5_{\gamma,\alpha} \quad (3r_T r_V N_v) \quad (7534)$$

$$\tau^7_{a,b} = \sum_{\gamma \in A} Y^1_{b,\gamma} \tau^6_{\gamma,a} \quad (2r_T N_v^2) \quad (7535)$$

$$\tau^8_{\gamma,a} = \sum_{b \in V} Y^1_{b,\gamma} \tau^7_{b,a} \quad (2r_T N_v^2) \quad (7536)$$

$$\tau^9_{\gamma,\delta,w} = \sum_{a \in V} {}^2D^1_{a,w} Y^{1,*}_{a,\delta} \tau^8_{\gamma,a} \quad (3r_D r_T^2 N_v) \quad (7537)$$

$$\tau^{10}_{\gamma,\delta,w} = \sum_{\epsilon \in A} Z_{\epsilon,\gamma} \tau^0_{\epsilon,\delta,w} \tau^9_{\epsilon,\delta,w} \quad (3r_D r_T^3) \quad (7538)$$

$$\tau^{11}_{\gamma,\delta,w} = \sum_{a \in V} {}^2D^3_{a,w} Y^3_{a,\gamma} Y^{3,*}_{a,\delta} \quad (3r_D r_T^2 N_v) \quad (7539)$$

$$\tau^{12}_{\gamma,\delta,w} = \sum_{i \in O} {}^2D^4_{i,w} Y^4_{i,\gamma} Y^{4,*}_{i,\delta} \quad (3r_D r_T^2 N_o) \quad (7540)$$

$${}^2R^z_{\gamma,\delta} \leftarrow - \sum_{\epsilon \in A} \sum_{w \in D} \frac{1}{2} \tau^{10}_{\epsilon,\gamma,w} \tau^{11}_{\epsilon,\delta,w} \tau^{12}_{\epsilon,\delta,w} \quad (3r_D r_T^3) \quad (7541)$$



Raw expression

$${}^2R^z_{\epsilon,\zeta} \leftarrow - \sum_{i \in O} \sum_{j \in O} \sum_{k \in O} \sum_{l \in O} \sum_{a \in V} \sum_{b \in V} \sum_{c \in V} \sum_{d \in V} \frac{1}{2} \quad (7542)$$

$$Y^{1,*}_{a,\epsilon} Y^{2,*}_{i,\epsilon} Y^{3,*}_{b,\zeta} Y^{4,*}_{j,\zeta}$$

$${}^2D^{a,i,b,j} {}^2T_{a,k,d,l} {}^2T_{c,i,b,j} V_{k,c,l,d}$$

Factorized expression

$$\tau^0_{\gamma,\alpha} = \sum_{a \in V} W^2_{a,\alpha} Y^1_{a,\gamma} \quad (2r_T r_V N_v) \quad (7543)$$

$$\tau^1_{\gamma,\alpha} = \sum_{a \in V} W^4_{a,\alpha} Y^3_{a,\gamma} \quad (2r_T r_V N_v) \quad (7544)$$

$$\tau^2_{\gamma,\alpha} = \sum_{i \in O} W^3_{i,\alpha} Y^4_{i,\gamma} \quad (2r_T r_V N_o) \quad (7545)$$

$$\tau^3_{\gamma,\alpha} = \sum_{\beta \in B} X_{\alpha,\beta} \tau^1_{\gamma,\beta} \tau^2_{\gamma,\beta} \quad (3r_T r_V^2) \quad (7546)$$

$$\tau^4_{\gamma,\alpha} = \sum_{\delta \in A} Z_{\gamma,\delta} \tau^3_{\delta,\alpha} \quad (2r_T^2 r_V) \quad (7547)$$

$$\tau^5_{\gamma,i} = \sum_{\alpha \in B} W^1_{i,\alpha} \tau^0_{\gamma,\alpha} \tau^4_{\gamma,\alpha} \quad (3r_T r_V N_o) \quad (7548)$$

$$\tau^6_{i,j} = \sum_{\gamma \in A} Y^2_{j,\gamma} \tau^5_{\gamma,i} \quad (2r_T N_o^2) \quad (7549)$$

$$\tau^7_{\gamma,i} = \sum_{j \in O} Y^2_{j,\gamma} \tau^6_{j,i} \quad (2r_T N_o^2) \quad (7550)$$

$$\tau^8_{\gamma,\delta,w} = \sum_{i \in O} {}^2D^2_{i,w} Y^{2,*}_{i,\delta} \tau^7_{\gamma,i} \quad (3r_D r_T^2 N_o) \quad (7551)$$

$$\tau^9_{\gamma,\delta,w} = \sum_{a \in V} {}^2D^1_{a,w} Y^1_{a,\gamma} Y^{1,*}_{a,\delta} \quad (3r_D r_T^2 N_v) \quad (7552)$$

$$\tau^{10}_{\gamma,\delta,w} = \sum_{a \in V} {}^2D^3_{a,w} Y^3_{a,\gamma} Y^{3,*}_{a,\delta} \quad (3r_D r_T^2 N_v) \quad (7553)$$

$$\tau^{11}_{\gamma,\delta,w} = \sum_{i \in O} {}^2D^4_{i,w} Y^4_{i,\gamma} Y^{4,*}_{i,\delta} \quad (3r_D r_T^2 N_o) \quad (7554)$$

$$\tau^{12}_{\gamma,\delta,w} = \sum_{\epsilon \in A} Z_{\gamma,\epsilon} \tau^{10}_{\epsilon,\delta,w} \tau^{11}_{\epsilon,\delta,w} \quad (3r_D r_T^3) \quad (7555)$$

$${}^2R^z_{\gamma,\delta} \leftarrow - \sum_{\epsilon \in A} \sum_{w \in D} \frac{1}{2} \tau^{12}_{\epsilon,\delta,w} \tau^8_{\epsilon,\gamma,w} \tau^9_{\epsilon,\gamma,w} \quad (3r_D r_T^3) \quad (7556)$$

Raw expression

$${}^2R^z_{\epsilon,\zeta} \leftarrow - \sum_{i \in O} \sum_{j \in O} \sum_{k \in O} \sum_{l \in O} \sum_{a \in V} \sum_{b \in V} \sum_{c \in V} \sum_{d \in V} \frac{1}{2} \quad (7557)$$

$$Y^{1,*}_{a,\epsilon} Y^{2,*}_{i,\epsilon} Y^{3,*}_{b,\zeta} Y^{4,*}_{j,\zeta}$$

$${}^2D^{a,i,b,j} {}^2T_{b,j,a,k} {}^2T_{c,i,d,l} V_{k,c,l,d}$$

Factorized expression

$$\tau^0_{\gamma,\delta,w} = \sum_{a \in V} {}^2D^1_{a,w} Y^3_{a,\gamma} Y^{1,*}_{a,\delta} \quad (3r_D r_T^2 N_v) \quad (7558)$$

$$\tau^1_{\gamma,\alpha} = \sum_{a \in V} W^2_{a,\alpha} Y^1_{a,\gamma} \quad (2r_T r_V N_v) \quad (7559)$$

$$\tau^2_{\gamma,\alpha} = \sum_{a \in V} W^4_{a,\alpha} Y^3_{a,\gamma} \quad (2r_T r_V N_v) \quad (7560)$$

$$\tau^3_{\gamma,\alpha} = \sum_{i \in O} W^3_{i,\alpha} Y^4_{i,\gamma} \quad (2r_T r_V N_o) \quad (7561)$$

$$\tau^4_{\gamma,\alpha} = \sum_{\beta \in B} X_{\alpha,\beta} \tau^2_{\gamma,\beta} \tau^3_{\gamma,\beta} \quad (3r_T r_V^2) \quad (7562)$$

$$\tau^5_{\gamma,\alpha} = \sum_{\delta \in A} Z_{\gamma,\delta} \tau^4_{\delta,\alpha} \quad (2r_T^2 r_V) \quad (7563)$$

$$\tau^6_{\gamma,i} = \sum_{\alpha \in B} W^1_{i,\alpha} \tau^1_{\gamma,\alpha} \tau^5_{\gamma,\alpha} \quad (3r_T r_V N_o) \quad (7564)$$

$$\tau^7_{i,j} = \sum_{\gamma \in A} Y^2_{j,\gamma} \tau^6_{\gamma,i} \quad (2r_T N_o^2) \quad (7565)$$

$$\tau^8_{\gamma,i} = \sum_{j \in O} Y^4_{j,\gamma} \tau^7_{j,i} \quad (2r_T N_o^2) \quad (7566)$$

$$\tau^9_{\gamma,\delta,w} = \sum_{i \in O} {}^2D^2_{i,w} Y^{2,*}_{i,\delta} \tau^8_{\gamma,i} \quad (3r_D r_T^2 N_o) \quad (7567)$$

$$\tau_{\gamma,\delta,w}^{10} = \sum_{\epsilon \in A} Z_{\gamma,\epsilon} \tau_{\epsilon,\delta,w}^0 \tau_{\epsilon,\delta,w}^9 \quad (3r_D r_T^3) \quad (7568)$$

$$\tau_{\gamma,\delta,i}^8 = \sum_{\epsilon \in A} Y_{i,\epsilon}^2 \tau_{\epsilon,\gamma,\delta}^7 \quad (2r_T^3 N_o) \quad (7581)$$

$$\tau_{\gamma,\delta,w}^{11} = \sum_{a \in V} {}^2D_{a,w}^3 Y_{a,\gamma}^1 Y_{a,\delta}^{3,*} \quad (3r_D r_T^2 N_v) \quad (7569)$$

$$\tau_{\gamma,\delta,w}^9 = \sum_{\epsilon \in A} \sum_{i \in O} {}^2D_{i,w}^2 Y_{i,\delta}^{2,*} \tau_{\epsilon,\delta,w}^0 \tau_{\gamma,\epsilon,i}^8 \quad (4r_D r_T^3 N_o) \quad (7582)$$

$$\tau_{\gamma,\delta,w}^{12} = \sum_{i \in O} {}^2D_{i,w}^4 Y_{i,\gamma}^2 Y_{i,\delta}^{4,*} \quad (3r_D r_T^2 N_o) \quad (7570)$$

$$\tau_{\gamma,\delta,w}^{10} = \sum_{a \in V} {}^2D_{a,w}^3 Y_{a,\gamma}^1 Y_{a,\delta}^{3,*} \quad (3r_D r_T^2 N_v) \quad (7583)$$

$${}^2R_{\gamma,\delta}^z \leftarrow - \sum_{\epsilon \in A} \sum_{w \in D} \frac{1}{2} \tau_{\epsilon,\gamma,w}^{10} \tau_{\epsilon,\delta,w}^{11} \tau_{\epsilon,\delta,w}^{12} \quad (3r_D r_T^3) \quad (7571)$$

$$\tau_{\gamma,\delta,w}^{11} = \sum_{i \in O} {}^2D_{i,w}^4 Y_{i,\gamma}^2 Y_{i,\delta}^{4,*} \quad (3r_D r_T^2 N_o) \quad (7584)$$

Raw expression

$${}^2R_{\epsilon,\zeta}^z \leftarrow - \sum_{i \in O} \sum_{j \in O} \sum_{k \in O} \sum_{l \in O} \sum_{a \in V} \sum_{b \in V} \sum_{c \in V} \sum_{d \in V} \frac{1}{2} \quad (7572)$$

$$Y_{a,\epsilon}^{1,*} Y_{i,\epsilon}^{2,*} Y_{b,\zeta}^{3,*} Y_{j,\zeta}^{4,*} {}^2D_{a,i,b,j} {}^2T_{b,j,a,l} {}^2T_{c,k,d,i} V_{l,d,k,c}$$

$${}^2R_{\gamma,\delta}^z \leftarrow - \sum_{\epsilon \in A} \sum_{w \in D} \frac{1}{2} \tau_{\epsilon,\delta,w}^{10} \tau_{\epsilon,\delta,w}^{11} \tau_{\epsilon,\gamma,w}^9 \quad (3r_D r_T^3) \quad (7585)$$

Raw expression

$${}^2R_{\epsilon,\zeta}^z \leftarrow - \sum_{i \in O} \sum_{j \in O} \sum_{k \in O} \sum_{l \in O} \sum_{a \in V} \sum_{b \in V} \sum_{c \in V} \sum_{d \in V} \frac{1}{2} \quad (7586)$$

$$Y_{a,\epsilon}^{1,*} Y_{i,\epsilon}^{2,*} Y_{b,\zeta}^{3,*} Y_{j,\zeta}^{4,*} {}^2D_{a,i,b,j} {}^2T_{b,j,c,i} {}^2T_{d,k,a,l} V_{k,d,l,c}$$

Factorized expression

$$\tau_{\gamma,\delta,w}^0 = \sum_{a \in V} {}^2D_{a,w}^1 Y_{a,\gamma}^3 Y_{a,\delta}^{1,*} \quad (3r_D r_T^2 N_v) \quad (7573)$$

Factorized expression

$$\tau_{\gamma,\alpha}^0 = \sum_{a \in V} W_{a,\alpha}^2 Y_{a,\gamma}^1 \quad (2r_T r_V N_v) \quad (7587)$$

$$\tau_{\gamma,\alpha}^1 = \sum_{a \in V} W_{a,\alpha}^4 Y_{a,\gamma}^3 \quad (2r_T r_V N_v) \quad (7574)$$

$$\tau_{\gamma,\alpha}^2 = \sum_{i \in O} W_{i,\alpha}^3 Y_{i,\gamma}^4 \quad (2r_T r_V N_o) \quad (7575)$$

$$\tau_{\gamma,\alpha}^1 = \sum_{i \in O} W_{i,\alpha}^1 Y_{i,\gamma}^2 \quad (2r_T r_V N_o) \quad (7588)$$

$$\tau_{\gamma,\alpha}^3 = \sum_{\beta \in B} X_{\alpha,\beta} \tau_{\gamma,\beta}^1 \tau_{\gamma,\beta}^2 \quad (3r_T r_V^2) \quad (7576)$$

$$\tau_{\gamma,\alpha}^2 = \sum_{\beta \in B} X_{\beta,\alpha} \tau_{\gamma,\beta}^0 \tau_{\gamma,\beta}^1 \quad (3r_T r_V^2) \quad (7589)$$

$$\tau_{\gamma,\alpha}^4 = \sum_{\delta \in A} Z_{\gamma,\delta} \tau_{\delta,\alpha}^3 \quad (2r_T^2 r_V) \quad (7577)$$

$$\tau_{\gamma,\alpha}^3 = \sum_{\delta \in A} Z_{\delta,\gamma} \tau_{\delta,\alpha}^2 \quad (2r_T^2 r_V) \quad (7590)$$

$$\tau_{\gamma,\alpha}^5 = \sum_{a \in V} W_{a,\alpha}^2 Y_{a,\gamma}^1 \quad (2r_T r_V N_v) \quad (7578)$$

$$\tau_{\gamma,\alpha}^4 = \sum_{i \in O} W_{i,\alpha}^3 Y_{i,\gamma}^4 \quad (2r_T r_V N_o) \quad (7591)$$

$$\tau_{\gamma,\delta,i}^6 = \sum_{\alpha \in B} W_{i,\alpha}^1 \tau_{\delta,\alpha}^4 \tau_{\gamma,\alpha}^5 \quad (3r_T^2 r_V N_o) \quad (7579)$$

$$\tau_{\gamma,a}^5 = \sum_{\alpha \in B} W_{a,\alpha}^4 \tau_{\gamma,\alpha}^3 \tau_{\gamma,\alpha}^4 \quad (3r_T r_V N_v) \quad (7592)$$

$$\tau_{\gamma,\delta,\epsilon}^7 = \sum_{i \in O} Z_{\gamma,\epsilon} Y_{i,\epsilon}^4 \tau_{\gamma,\delta,i}^6 \quad (3r_T^3 N_o) \quad (7580)$$

$$\tau_{\gamma,\delta}^6 = \sum_{a \in V} Y_{a,\delta}^3 \tau_{\gamma,a}^5 \quad (2r_T^2 N_v) \quad (7593)$$

$$\tau^7_{\gamma,a} = \sum_{\delta \in A} Y^3_{a,\delta} \tau^6_{\delta,\gamma} \quad (2r_T^2 N_v) \quad (7594)$$

$$\tau^5_{\gamma,\alpha} = \sum_{i \in O} W^1_{i,\alpha} Y^2_{i,\gamma} \quad (2r_T r_V N_o) \quad (7607)$$

$$\tau^8_{\gamma,\delta,w} = \sum_{a \in V} {}^2D^1_{a,w} Y^{1,*}_{a,\delta} \tau^7_{\gamma,a} \quad (3r_D r_T^2 N_v) \quad (7595)$$

$$\tau^6_{\gamma,\alpha} = \sum_{\beta \in B} X_{\beta,\alpha} \tau^4_{\gamma,\beta} \tau^5_{\gamma,\beta} \quad (3r_T r_V^2) \quad (7608)$$

$$\tau^9_{\gamma,\delta,w} = \sum_{i \in O} {}^2D^2_{i,w} Y^4_{i,\gamma} Y^{2,*}_{i,\delta} \quad (3r_D r_T^2 N_o) \quad (7596)$$

$$\tau^7_{\gamma,\alpha} = \sum_{\delta \in A} Z_{\delta,\gamma} \tau^6_{\delta,\alpha} \quad (2r_T^2 r_V) \quad (7609)$$

$$\tau^{10}_{\gamma,\delta,w} = \sum_{\epsilon \in A} Z_{\gamma,\epsilon} \tau^8_{\epsilon,\delta,w} \tau^9_{\epsilon,\delta,w} \quad (3r_D r_T^3) \quad (7597)$$

$$\tau^8_{\gamma,\delta,i} = \sum_{\alpha \in B} W^3_{i,\alpha} \tau^3_{\delta,\alpha} \tau^7_{\gamma,\alpha} \quad (3r_T^2 r_V N_o) \quad (7610)$$

$$\tau^{11}_{\gamma,\delta,w} = \sum_{a \in V} {}^2D^3_{a,w} Y^1_{a,\gamma} Y^{3,*}_{a,\delta} \quad (3r_D r_T^2 N_v) \quad (7598)$$

$$\tau^9_{\gamma,\delta,\epsilon} = \sum_{i \in O} Y^2_{i,\gamma} \tau^8_{\delta,\epsilon,i} \quad (2r_T^3 N_o) \quad (7611)$$

$$\tau^{12}_{\gamma,\delta,w} = \sum_{i \in O} {}^2D^4_{i,w} Y^2_{i,\gamma} Y^{4,*}_{i,\delta} \quad (3r_D r_T^2 N_o) \quad (7599)$$

$$\tau^{10}_{\gamma,\delta,i} = \sum_{\epsilon \in A} Z_{\gamma,\epsilon} Y^4_{i,\epsilon} \tau^9_{\gamma,\delta,\epsilon} \quad (3r_T^3 N_o) \quad (7612)$$

$${}^2R^z_{\gamma,\delta} \leftarrow - \sum_{\epsilon \in A} \sum_{w \in D} \frac{1}{2} \tau^{10}_{\epsilon,\gamma,w} \tau^{11}_{\epsilon,\delta,w} \tau^{12}_{\epsilon,\delta,w} \quad (3r_D r_T^3) \quad (7600)$$

$$\tau^{11}_{\gamma,\delta,w} = \sum_{\epsilon \in A} \sum_{i \in O} {}^2D^4_{i,w} Y^{4,*}_{i,\delta} \tau^{10}_{\epsilon,\gamma,i} \tau^2_{\epsilon,\delta,w} \quad (4r_D r_T^3 N_o) \quad (7613)$$

Raw expression

$${}^2R^z_{\gamma,\delta} \leftarrow - \sum_{\epsilon \in A} \sum_{w \in D} \frac{1}{2} \tau^0_{\epsilon,\gamma,w} \tau^1_{\epsilon,\gamma,w} \tau^{11}_{\epsilon,\delta,w} \quad (3r_D r_T^3) \quad (7614)$$

$${}^2R^z_{\epsilon,\zeta} \leftarrow - \sum_{i \in O} \sum_{j \in O} \sum_{k \in O} \sum_{l \in O} \sum_{a \in V} \sum_{b \in V} \sum_{c \in V} \sum_{d \in V} \frac{1}{2} Y^{1,*}_{a,\epsilon} Y^{2,*}_{i,\epsilon} Y^{3,*}_{b,\zeta} Y^{4,*}_{j,\zeta} {}^2D^{a,i,b,j} {}^2T_{b,j,c,l} {}^2T_{d,k,a,i} V_{k,c,l,d} \quad (7601)$$

Raw expression

$${}^2R^z_{\epsilon,\zeta} \leftarrow - \sum_{i \in O} \sum_{j \in O} \sum_{k \in O} \sum_{l \in O} \sum_{a \in V} \sum_{b \in V} \sum_{c \in V} \sum_{d \in V} \frac{1}{2} Y^{1,*}_{a,\epsilon} Y^{2,*}_{i,\epsilon} Y^{3,*}_{b,\zeta} Y^{4,*}_{j,\zeta} {}^2D^{a,i,b,j} {}^2T_{b,j,d,l} {}^2T_{c,i,a,k} V_{k,c,l,d} \quad (7615)$$

Factorized expression

Factorized expression

$$\tau^0_{\gamma,\delta,w} = \sum_{a \in V} {}^2D^1_{a,w} Y^3_{a,\gamma} Y^{1,*}_{a,\delta} \quad (3r_D r_T^2 N_v) \quad (7602)$$

$$\tau^0_{\gamma,\alpha} = \sum_{a \in V} W^2_{a,\alpha} Y^3_{a,\gamma} \quad (2r_T r_V N_v) \quad (7616)$$

$$\tau^1_{\gamma,\delta,w} = \sum_{i \in O} {}^2D^2_{i,w} Y^4_{i,\gamma} Y^{2,*}_{i,\delta} \quad (3r_D r_T^2 N_o) \quad (7603)$$

$$\tau^1_{\gamma,\alpha,i} = \sum_{\beta \in B} W^1_{i,\beta} X_{\beta,\alpha} \tau^0_{\gamma,\beta} \quad (3r_T r_V^2 N_o) \quad (7617)$$

$$\tau^2_{\gamma,\delta,w} = \sum_{a \in V} {}^2D^3_{a,w} Y^1_{a,\gamma} Y^{3,*}_{a,\delta} \quad (3r_D r_T^2 N_v) \quad (7604)$$

$$\tau^2_{\gamma,\alpha} = \sum_{i \in O} W^3_{i,\alpha} Y^4_{i,\gamma} \quad (2r_T r_V N_o) \quad (7618)$$

$$\tau^3_{\gamma,\alpha} = \sum_{a \in V} W^4_{a,\alpha} Y^3_{a,\gamma} \quad (2r_T r_V N_v) \quad (7605)$$

$$\tau^4_{\gamma,\alpha} = \sum_{a \in V} W^2_{a,\alpha} Y^1_{a,\gamma} \quad (2r_T r_V N_v) \quad (7606)$$

$$\tau^3_{\gamma,\alpha} = \sum_{a \in V} W^4_{a,\alpha} Y^1_{a,\gamma} \quad (2r_T r_V N_v) \quad (7619)$$

$$\tau_{\gamma,\delta,i}^4 = \sum_{\alpha \in B} \tau_{\delta,\alpha}^2 \tau_{\gamma,\alpha}^3 \tau_{\delta,\alpha,i}^1 \quad (3r_T^2 r_V N_o) \quad (7620)$$

$$\tau_{\gamma,\alpha}^2 = \sum_{i \in O} W_{i,\alpha}^3 Y_{i,\gamma}^2 \quad (2r_T r_V N_o) \quad (7633)$$

$$\tau_{\gamma,\delta}^5 = \sum_{i \in O} Y_{i,\gamma}^2 \tau_{\gamma,\delta,i}^4 \quad (2r_T^2 N_o) \quad (7621)$$

$$\tau_{\gamma,\alpha}^3 = \sum_{\beta \in B} X_{\alpha,\beta} \tau_{\gamma,\beta}^1 \tau_{\gamma,\beta}^2 \quad (3r_T r_V^2) \quad (7634)$$

$$\tau_{\gamma,\delta}^6 = \sum_{\epsilon \in A} Z_{\delta,\epsilon} \tau_{\gamma,\epsilon}^5 \quad (2r_T^3) \quad (7622)$$

$$\tau_{\gamma,\alpha}^4 = \sum_{\delta \in A} Z_{\delta,\gamma} \tau_{\delta,\alpha}^3 \quad (2r_T^2 r_V) \quad (7635)$$

$$\tau_{\gamma,\delta}^7 = \sum_{\epsilon \in A} Z_{\epsilon,\delta} \tau_{\epsilon,\gamma}^6 \quad (2r_T^3) \quad (7623)$$

$$\tau_{\gamma,\alpha}^5 = \sum_{a \in V} W_{a,\alpha}^2 Y_{a,\gamma}^3 \quad (2r_T r_V N_v) \quad (7636)$$

$$\tau_{\gamma,\delta,w}^8 = \sum_{a \in V} {}^2D_{a,w}^1 Y_{a,\gamma}^3 Y_{a,\delta}^{1,*} \quad (3r_D r_T^2 N_v) \quad (7624)$$

$$\tau_{\gamma,i}^6 = \sum_{\alpha \in B} W_{i,\alpha}^1 \tau_{\gamma,\alpha}^4 \tau_{\gamma,\alpha}^5 \quad (3r_T r_V N_o) \quad (7637)$$

$$\tau_{\gamma,\delta,w}^9 = \sum_{i \in O} {}^2D_{i,w}^2 Y_{i,\gamma}^4 Y_{i,\delta}^{2,*} \quad (3r_D r_T^2 N_o) \quad (7625)$$

$$\tau_{i,j}^7 = \sum_{\gamma \in A} Y_{j,\gamma}^4 \tau_{\gamma,i}^6 \quad (2r_T N_o^2) \quad (7638)$$

$$\tau_{\gamma,\delta,w}^{10} = \sum_{\epsilon \in A} \tau_{\gamma,\epsilon}^7 \tau_{\epsilon,\delta,w}^8 \tau_{\epsilon,\delta,w}^9 \quad (3r_D r_T^3) \quad (7626)$$

$$\tau_{\gamma,i}^8 = \sum_{j \in O} Y_{j,\gamma}^4 \tau_{j,i}^7 \quad (2r_T N_o^2) \quad (7639)$$

$$\tau_{\gamma,\delta,w}^{11} = \sum_{a \in V} {}^2D_{a,w}^3 Y_{a,\gamma}^1 Y_{a,\delta}^{3,*} \quad (3r_D r_T^2 N_v) \quad (7627)$$

$$\tau_{\gamma,\delta,w}^9 = \sum_{i \in O} {}^2D_{i,w}^2 Y_{i,\gamma}^{2,*} \tau_{i,\delta}^8 \tau_{\gamma,i}^8 \quad (3r_D r_T^2 N_o) \quad (7640)$$

$$\tau_{\gamma,\delta,w}^{12} = \sum_{i \in O} {}^2D_{i,w}^4 Y_{i,\gamma}^2 Y_{i,\delta}^{4,*} \quad (3r_D r_T^2 N_o) \quad (7628)$$

$$\tau_{\gamma,\delta,w}^{10} = \sum_{\epsilon \in A} Z_{\gamma,\epsilon} \tau_{\epsilon,\delta,w}^0 \tau_{\epsilon,\delta,w}^9 \quad (3r_D r_T^3) \quad (7641)$$

$${}^2R_{\gamma,\delta}^z \leftarrow - \sum_{\epsilon \in A} \sum_{w \in D} \frac{1}{2} \tau_{\epsilon,\gamma,w}^{10} \tau_{\epsilon,\delta,w}^{11} \tau_{\epsilon,\delta,w}^{12} \quad (3r_D r_T^3) \quad (7629)$$

$$\tau_{\gamma,\delta,w}^{11} = \sum_{a \in V} {}^2D_{a,w}^3 Y_{a,\gamma}^1 Y_{a,\delta}^{3,*} \quad (3r_D r_T^2 N_v) \quad (7642)$$

Raw expression

$${}^2R_{\epsilon,\zeta}^z \leftarrow - \sum_{i \in O} \sum_{j \in O} \sum_{k \in O} \sum_{l \in O} \sum_{a \in V} \sum_{b \in V} \sum_{c \in V} \sum_{d \in V} \frac{1}{2} \quad (7630)$$

$$Y_{a,\epsilon}^{1,*} Y_{i,\epsilon}^{2,*} Y_{b,\zeta}^{3,*} Y_{j,\zeta}^{4,*} {}^2D_{a,i,b,j} {}^2T_{b,k,a,i} {}^2T_{c,j,d,l} V_{k,c,l,d}$$

$$\tau_{\gamma,\delta,w}^{12} = \sum_{i \in O} {}^2D_{i,w}^4 Y_{i,\gamma}^2 Y_{i,\delta}^{4,*} \quad (3r_D r_T^2 N_o) \quad (7643)$$

$${}^2R_{\gamma,\delta}^z \leftarrow - \sum_{\epsilon \in A} \sum_{w \in D} \frac{1}{2} \tau_{\epsilon,\gamma,w}^{10} \tau_{\epsilon,\delta,w}^{11} \tau_{\epsilon,\delta,w}^{12} \quad (3r_D r_T^3) \quad (7644)$$

Factorized expression

$$\tau_{\gamma,\delta,w}^0 = \sum_{a \in V} {}^2D_{a,w}^1 Y_{a,\gamma}^3 Y_{a,\delta}^{1,*} \quad (3r_D r_T^2 N_v) \quad (7631)$$

$$\tau_{\gamma,\alpha}^1 = \sum_{a \in V} W_{a,\alpha}^4 Y_{a,\gamma}^1 \quad (2r_T r_V N_v) \quad (7632)$$

Raw expression

$${}^2R_{\epsilon,\zeta}^z \leftarrow - \sum_{i \in O} \sum_{j \in O} \sum_{k \in O} \sum_{l \in O} \sum_{a \in V} \sum_{b \in V} \sum_{c \in V} \sum_{d \in V} \frac{1}{2} \quad (7645)$$

$$Y_{a,\epsilon}^{1,*} Y_{i,\epsilon}^{2,*} Y_{b,\zeta}^{3,*} Y_{j,\zeta}^{4,*} {}^2D_{a,i,b,j} {}^2T_{b,k,a,i} {}^2T_{c,l,d,j} V_{k,d,l,c}$$

Factorized expression

$$\tau_{\gamma,\delta,w}^0 = \sum_{a \in V} {}^2D_{a,w}^1 Y_{a,\gamma}^3 Y_{a,\delta}^{1,*} \quad (3r_D r_T^2 N_v) \quad (7646)$$

$$\tau_{\gamma,\delta,w}^1 = \sum_{i \in O} {}^2D_{i,w}^2 Y_{i,\gamma}^4 Y_{i,\delta}^{2,*} \quad (3r_D r_T^2 N_o) \quad (7647)$$

$$\tau_{\gamma,\delta,w}^2 = \sum_{\epsilon \in A} Z_{\gamma,\epsilon} \tau_{\epsilon,\delta,w}^0 \tau_{\epsilon,\delta,w}^1 \quad (3r_D r_T^3) \quad (7648)$$

$$\tau_{\gamma,\alpha}^3 = \sum_{a \in V} W_{a,\alpha}^4 Y_{a,\gamma}^1 \quad (2r_T r_V N_v) \quad (7649)$$

$$\tau_{\gamma,\alpha}^4 = \sum_{i \in O} W_{i,\alpha}^3 Y_{i,\gamma}^2 \quad (2r_T r_V N_o) \quad (7650)$$

$$\tau_{\gamma,\alpha}^5 = \sum_{\beta \in B} X_{\alpha,\beta} \tau_{\gamma,\beta}^3 \tau_{\gamma,\beta}^4 \quad (3r_T r_V^2) \quad (7651)$$

$$\tau_{\gamma,\alpha}^6 = \sum_{\delta \in A} Z_{\delta,\gamma} \tau_{\delta,\alpha}^5 \quad (2r_T^2 r_V) \quad (7652)$$

$$\tau_{\gamma,\alpha}^7 = \sum_{a \in V} W_{a,\alpha}^2 Y_{a,\gamma}^3 \quad (2r_T r_V N_v) \quad (7653)$$

$$\tau_{\gamma,i}^8 = \sum_{\alpha \in B} W_{i,\alpha}^1 \tau_{\gamma,\alpha}^6 \tau_{\gamma,\alpha}^7 \quad (3r_T r_V N_o) \quad (7654)$$

$$\tau_{i,j}^9 = \sum_{\gamma \in A} Y_{j,\gamma}^4 \tau_{\gamma,i}^8 \quad (2r_T N_o^2) \quad (7655)$$

$$\tau_{\gamma,i}^{10} = \sum_{j \in O} Y_{j,\gamma}^2 \tau_{j,i}^9 \quad (2r_T N_o^2) \quad (7656)$$

$$\tau_{\gamma,\delta,w}^{11} = \sum_{i \in O} {}^2D_{i,w}^4 Y_{i,\delta}^{4,*} \tau_{\gamma,i}^{10} \quad (3r_D r_T^2 N_o) \quad (7657)$$

$$\tau_{\gamma,\delta,w}^{12} = \sum_{a \in V} {}^2D_{a,w}^3 Y_{a,\gamma}^1 Y_{a,\delta}^{3,*} \quad (3r_D r_T^2 N_v) \quad (7658)$$

$${}^2R_{\gamma,\delta}^z \leftarrow - \sum_{\epsilon \in A} \sum_{w \in D} \frac{1}{2} \tau_{\epsilon,\delta,w}^{11} \tau_{\epsilon,\delta,w}^{12} \tau_{\epsilon,\gamma,w}^2 \quad (3r_D r_T^3) \quad (7659)$$

Raw expression

$${}^2R_{\epsilon,\zeta}^z \leftarrow - \sum_{i \in O} \sum_{j \in O} \sum_{k \in O} \sum_{l \in O} \sum_{a \in V} \sum_{b \in V} \sum_{c \in V} \sum_{d \in V} \frac{1}{2} Y_{a,\epsilon}^{1,*} Y_{i,\epsilon}^{2,*} Y_{b,\zeta}^{3,*} Y_{j,\zeta}^{4,*} {}^2D_{a,i,b,j} {}^2T_{b,k,d,l} {}^2T_{c,j,a,i} V_{k,c,l,d} \quad (7660)$$

Factorized expression

$$\tau_{\gamma,\delta,w}^0 = \sum_{a \in V} {}^2D_{a,w}^1 Y_{a,\gamma}^3 Y_{a,\delta}^{1,*} \quad (3r_D r_T^2 N_v) \quad (7661)$$

$$\tau_{\gamma,\delta,w}^1 = \sum_{i \in O} {}^2D_{i,w}^2 Y_{i,\gamma}^4 Y_{i,\delta}^{2,*} \quad (3r_D r_T^2 N_o) \quad (7662)$$

$$\tau_{\gamma,\delta,w}^2 = \sum_{i \in O} {}^2D_{i,w}^4 Y_{i,\gamma}^2 Y_{i,\delta}^{4,*} \quad (3r_D r_T^2 N_o) \quad (7663)$$

$$\tau_{\gamma,\alpha}^3 = \sum_{i \in O} W_{i,\alpha}^1 Y_{i,\gamma}^2 \quad (2r_T r_V N_o) \quad (7664)$$

$$\tau_{\gamma,\alpha}^4 = \sum_{a \in V} W_{a,\alpha}^4 Y_{a,\gamma}^3 \quad (2r_T r_V N_v) \quad (7665)$$

$$\tau_{\gamma,\alpha}^5 = \sum_{i \in O} W_{i,\alpha}^3 Y_{i,\gamma}^4 \quad (2r_T r_V N_o) \quad (7666)$$

$$\tau_{\gamma,\alpha}^6 = \sum_{\beta \in B} X_{\alpha,\beta} \tau_{\gamma,\beta}^4 \tau_{\gamma,\beta}^5 \quad (3r_T r_V^2) \quad (7667)$$

$$\tau_{\gamma,\alpha}^7 = \sum_{\delta \in A} Z_{\gamma,\delta} \tau_{\delta,\alpha}^6 \quad (2r_T^2 r_V) \quad (7668)$$

$$\tau_{\gamma,a}^8 = \sum_{\alpha \in B} W_{a,\alpha}^2 \tau_{\gamma,\alpha}^3 \tau_{\gamma,\alpha}^7 \quad (3r_T r_V N_v) \quad (7669)$$

$$\tau_{a,b}^9 = \sum_{\gamma \in A} Y_{b,\gamma}^1 \tau_{\gamma,a}^8 \quad (2r_T N_v^2) \quad (7670)$$

$$\tau_{\gamma,a}^{10} = \sum_{b \in V} Y_{b,\gamma}^1 \tau_{b,a}^9 \quad (2r_T N_v^2) \quad (7671)$$

$$\tau_{\gamma,\delta,w}^{11} = \sum_{a \in V} {}^2D_{a,w}^3 Y_{a,\delta}^{3,*} \tau_{\gamma,a}^{10} \quad (3r_D r_T^2 N_v) \quad (7672)$$

$$\tau_{\gamma,\delta,w}^{12} = \sum_{\epsilon \in A} Z_{\epsilon,\gamma} \tau_{\epsilon,\delta,w}^{11} \tau_{\epsilon,\delta,w}^2 \quad (3r_D r_T^3) \quad (7673)$$

$${}^2R^z_{\gamma,\delta} \leftarrow - \sum_{\epsilon \in A} \sum_{w \in D} \frac{1}{2} \tau^0_{\epsilon,\gamma,w} \tau^1_{\epsilon,\gamma,w} \tau^{12}_{\epsilon,\delta,w} \quad (3r_D r_T^3) \quad (7674)$$

Raw expression

$${}^2R^z_{\epsilon,\zeta} \leftarrow - \sum_{i \in O} \sum_{j \in O} \sum_{k \in O} \sum_{l \in O} \sum_{a \in V} \sum_{b \in V} \sum_{c \in V} \sum_{d \in V} \frac{1}{2} \quad (7675)$$

$$Y^{1,*}_{a,\epsilon} Y^{2,*}_{i,\epsilon} Y^{3,*}_{b,\zeta} Y^{4,*}_{j,\zeta}$$

$${}^2D^{a,i,b,j} {}^2T_{b,l,d,j} {}^2T_{c,k,a,i} V_{k,c,l,d}$$

Factorized expression

$$\tau^0_{\gamma,\alpha} = \sum_{a \in V} W^2_{a,\alpha} Y^1_{a,\gamma} \quad (2r_T r_V N_v) \quad (7676)$$

$$\tau^1_{\gamma,\alpha} = \sum_{a \in V} W^4_{a,\alpha} Y^3_{a,\gamma} \quad (2r_T r_V N_v) \quad (7677)$$

$$\tau^2_{\gamma,\alpha} = \sum_{i \in O} W^3_{i,\alpha} Y^4_{i,\gamma} \quad (2r_T r_V N_o) \quad (7678)$$

$$\tau^3_{\gamma,\alpha} = \sum_{\beta \in B} X_{\alpha,\beta} \tau^1_{\gamma,\beta} \tau^2_{\gamma,\beta} \quad (3r_T r_V^2) \quad (7679)$$

$$\tau^4_{\gamma,\alpha} = \sum_{\delta \in A} Z_{\gamma,\delta} \tau^3_{\delta,\alpha} \quad (2r_T^2 r_V) \quad (7680)$$

$$\tau^5_{\gamma,i} = \sum_{\alpha \in B} W^1_{i,\alpha} \tau^0_{\gamma,\alpha} \tau^4_{\gamma,\alpha} \quad (3r_T r_V N_o) \quad (7681)$$

$$\tau^6_{i,j} = \sum_{\gamma \in A} Y^2_{j,\gamma} \tau^5_{\gamma,i} \quad (2r_T N_o^2) \quad (7682)$$

$$\tau^7_{\gamma,i} = \sum_{j \in O} Y^2_{j,\gamma} \tau^6_{j,i} \quad (2r_T N_o^2) \quad (7683)$$

$$\tau^8_{\gamma,\delta,w} = \sum_{i \in O} {}^2D^4_{i,w} Y^{4,*}_{i,\delta} \tau^7_{\gamma,i} \quad (3r_D r_T^2 N_o) \quad (7684)$$

$$\tau^9_{\gamma,\delta,w} = \sum_{a \in V} {}^2D^3_{a,w} Y^1_{a,\gamma} Y^{3,*}_{a,\delta} \quad (3r_D r_T^2 N_v) \quad (7685)$$

$$\tau^{10}_{\gamma,\delta,w} = \sum_{a \in V} {}^2D^1_{a,w} Y^3_{a,\gamma} Y^{1,*}_{a,\delta} \quad (3r_D r_T^2 N_v) \quad (7686)$$

$$\tau^{11}_{\gamma,\delta,w} = \sum_{i \in O} {}^2D^2_{i,w} Y^4_{i,\gamma} Y^{2,*}_{i,\delta} \quad (3r_D r_T^2 N_o) \quad (7687)$$

$$\tau^{12}_{\gamma,\delta,w} = \sum_{\epsilon \in A} Z_{\gamma,\epsilon} \tau^{10}_{\epsilon,\delta,w} \tau^{11}_{\epsilon,\delta,w} \quad (3r_D r_T^3) \quad (7688)$$

$${}^2R^z_{\gamma,\delta} \leftarrow - \sum_{\epsilon \in A} \sum_{w \in D} \frac{1}{2} \tau^{12}_{\epsilon,\gamma,w} \tau^8_{\epsilon,\delta,w} \tau^9_{\epsilon,\delta,w} \quad (3r_D r_T^3) \quad (7689)$$

Raw expression

$${}^2R^z_{\epsilon,\zeta} \leftarrow - \sum_{i \in O} \sum_{j \in O} \sum_{k \in O} \sum_{l \in O} \sum_{a \in V} \sum_{b \in V} \sum_{c \in V} \sum_{d \in V} \frac{1}{2} \quad (7690)$$

$$Y^{1,*}_{a,\epsilon} Y^{2,*}_{i,\epsilon} Y^{3,*}_{b,\zeta} Y^{4,*}_{j,\zeta}$$

$${}^2D^{a,i,b,j} {}^2T_{c,i,a,l} {}^2T_{d,k,b,j} V_{l,c,k,d}$$

Factorized expression

$$\tau^0_{\gamma,\delta,w} = \sum_{a \in V} {}^2D^1_{a,w} Y^3_{a,\gamma} Y^{1,*}_{a,\delta} \quad (3r_D r_T^2 N_v) \quad (7691)$$

$$\tau^1_{\gamma,\alpha} = \sum_{a \in V} W^2_{a,\alpha} Y^1_{a,\gamma} \quad (2r_T r_V N_v) \quad (7692)$$

$$\tau^2_{\gamma,\alpha} = \sum_{a \in V} W^4_{a,\alpha} Y^1_{a,\gamma} \quad (2r_T r_V N_v) \quad (7693)$$

$$\tau^3_{\gamma,\alpha} = \sum_{i \in O} W^3_{i,\alpha} Y^2_{i,\gamma} \quad (2r_T r_V N_o) \quad (7694)$$

$$\tau^4_{\gamma,\alpha} = \sum_{\beta \in B} X_{\alpha,\beta} \tau^2_{\gamma,\beta} \tau^3_{\gamma,\beta} \quad (3r_T r_V^2) \quad (7695)$$

$$\tau^5_{\gamma,\alpha} = \sum_{\delta \in A} Z_{\delta,\gamma} \tau^4_{\delta,\alpha} \quad (2r_T^2 r_V) \quad (7696)$$

$$\tau^6_{\gamma,\delta,i} = \sum_{\alpha \in B} W^1_{i,\alpha} \tau^1_{\gamma,\alpha} \tau^5_{\delta,\alpha} \quad (3r_T^2 r_V N_o) \quad (7697)$$

$$\tau^7_{\gamma,\delta,\epsilon} = \sum_{i \in O} Z_{\gamma,\delta} Y^4_{i,\delta} \tau^6_{\gamma,\epsilon,i} \quad (3r_T^3 N_o) \quad (7698)$$

$$\tau^8_{\gamma,\delta,i} = \sum_{\epsilon \in A} Y^2_{i,\epsilon} \tau^7_{\epsilon,\gamma,\delta} \quad (2r_T^3 N_o) \quad (7699)$$

$$\tau_{\gamma,\delta,w}^9 = \sum_{\epsilon \in A} \sum_{i \in O} {}^2D^2_{i,w} Y^{2,*}_{i,\delta} \tau_{\epsilon,\delta,w}^0 \tau_{\epsilon,\gamma,i}^8 \quad (4r_D r_T^3 N_o) \quad (7700)$$

$$\tau_{\gamma,\delta,w}^{10} = \sum_{a \in V} {}^2D^3_{a,w} Y^3_{a,\gamma} Y^{3,*}_{a,\delta} \quad (3r_D r_T^2 N_v) \quad (7701)$$

$$\tau_{\gamma,\delta,w}^{11} = \sum_{i \in O} {}^2D^4_{i,w} Y^4_{i,\gamma} Y^{4,*}_{i,\delta} \quad (3r_D r_T^2 N_o) \quad (7702)$$

$${}^2R^z_{\gamma,\delta} \leftarrow - \sum_{\epsilon \in A} \sum_{w \in D} \frac{1}{2} \tau_{\epsilon,\delta,w}^{10} \tau_{\epsilon,\delta,w}^{11} \tau_{\epsilon,\gamma,w}^9 \quad (3r_D r_T^3) \quad (7703)$$

Raw expression

$${}^2R^z_{\epsilon,\zeta} \leftarrow - \sum_{i \in O} \sum_{j \in O} \sum_{k \in O} \sum_{l \in O} \sum_{a \in V} \sum_{b \in V} \sum_{c \in V} \sum_{d \in V} \frac{1}{2} \quad (7704)$$

$$Y^{1,*}_{a,\epsilon} Y^{2,*}_{i,\epsilon} Y^{3,*}_{b,\zeta} Y^{4,*}_{j,\zeta} {}^2D^{a,i,b,j} {}^2T_{c,i,b,j} {}^2T_{d,k,a,l} V_{k,d,l,c}$$

Factorized expression

$$\tau_{\gamma,\delta,w}^0 = \sum_{i \in O} {}^2D^2_{i,w} Y^2_{i,\gamma} Y^{2,*}_{i,\delta} \quad (3r_D r_T^2 N_o) \quad (7705)$$

$$\tau_{\gamma,\alpha}^1 = \sum_{a \in V} W^2_{a,\alpha} Y^1_{a,\gamma} \quad (2r_T r_V N_v) \quad (7706)$$

$$\tau_{\gamma,\alpha}^2 = \sum_{i \in O} W^1_{i,\alpha} Y^2_{i,\gamma} \quad (2r_T r_V N_o) \quad (7707)$$

$$\tau_{\gamma,\alpha}^3 = \sum_{\beta \in B} X_{\beta,\alpha} \tau_{\gamma,\beta}^1 \tau_{\gamma,\beta}^2 \quad (3r_T r_V^2) \quad (7708)$$

$$\tau_{\gamma,\alpha}^4 = \sum_{\delta \in A} Z_{\delta,\gamma} \tau_{\delta,\alpha}^3 \quad (2r_T^2 r_V) \quad (7709)$$

$$\tau_{\gamma,\alpha}^5 = \sum_{i \in O} W^3_{i,\alpha} Y^4_{i,\gamma} \quad (2r_T r_V N_o) \quad (7710)$$

$$\tau_{\gamma,a}^6 = \sum_{\alpha \in B} W^4_{a,\alpha} \tau_{\gamma,\alpha}^4 \tau_{\gamma,\alpha}^5 \quad (3r_T r_V N_v) \quad (7711)$$

$$\tau_{\gamma,\delta}^7 = \sum_{a \in V} Y^1_{a,\gamma} \tau_{\delta,a}^6 \quad (2r_T^2 N_v) \quad (7712)$$

$$\tau_{\gamma,a}^8 = \sum_{\delta \in A} Y^3_{a,\delta} \tau_{\gamma,\delta}^7 \quad (2r_T^2 N_v) \quad (7713)$$

$$\tau_{\gamma,\delta,w}^9 = \sum_{a \in V} {}^2D^1_{a,w} Y^{1,*}_{a,\delta} \tau_{\gamma,a}^8 \quad (3r_D r_T^2 N_v) \quad (7714)$$

$$\tau_{\gamma,\delta,w}^{10} = \sum_{\epsilon \in A} Z_{\epsilon,\gamma} \tau_{\epsilon,\delta,w}^0 \tau_{\epsilon,\delta,w}^9 \quad (3r_D r_T^3) \quad (7715)$$

$$\tau_{\gamma,\delta,w}^{11} = \sum_{a \in V} {}^2D^3_{a,w} Y^3_{a,\gamma} Y^{3,*}_{a,\delta} \quad (3r_D r_T^2 N_v) \quad (7716)$$

$$\tau_{\gamma,\delta,w}^{12} = \sum_{i \in O} {}^2D^4_{i,w} Y^4_{i,\gamma} Y^{4,*}_{i,\delta} \quad (3r_D r_T^2 N_o) \quad (7717)$$

$${}^2R^z_{\gamma,\delta} \leftarrow - \sum_{\epsilon \in A} \sum_{w \in D} \frac{1}{2} \tau_{\epsilon,\gamma,w}^{10} \tau_{\epsilon,\delta,w}^{11} \tau_{\epsilon,\delta,w}^{12} \quad (3r_D r_T^3) \quad (7718)$$

Raw expression

$${}^2R^z_{\epsilon,\zeta} \leftarrow - \sum_{i \in O} \sum_{j \in O} \sum_{k \in O} \sum_{l \in O} \sum_{a \in V} \sum_{b \in V} \sum_{c \in V} \sum_{d \in V} \frac{1}{2} \quad (7719)$$

$$Y^{1,*}_{a,\epsilon} Y^{2,*}_{i,\epsilon} Y^{3,*}_{b,\zeta} Y^{4,*}_{j,\zeta} {}^2D^{a,i,b,j} {}^2T_{c,j,a,i} {}^2T_{d,k,b,l} V_{k,d,l,c}$$

Factorized expression

$$\tau_{\gamma,\delta,w}^0 = \sum_{a \in V} {}^2D^1_{a,w} Y^3_{a,\gamma} Y^{1,*}_{a,\delta} \quad (3r_D r_T^2 N_v) \quad (7720)$$

$$\tau_{\gamma,\delta,w}^1 = \sum_{i \in O} {}^2D^2_{i,w} Y^4_{i,\gamma} Y^{2,*}_{i,\delta} \quad (3r_D r_T^2 N_o) \quad (7721)$$

$$\tau_{\gamma,\delta,w}^2 = \sum_{i \in O} {}^2D^4_{i,w} Y^2_{i,\gamma} Y^{4,*}_{i,\delta} \quad (3r_D r_T^2 N_o) \quad (7722)$$

$$\tau_{\gamma,\alpha}^3 = \sum_{a \in V} W^2_{a,\alpha} Y^1_{a,\gamma} \quad (2r_T r_V N_v) \quad (7723)$$

$$\tau_{\gamma,\alpha}^4 = \sum_{i \in O} W^1_{i,\alpha} Y^2_{i,\gamma} \quad (2r_T r_V N_o) \quad (7724)$$

$$\tau_{\gamma,\alpha}^5 = \sum_{\beta \in B} X_{\beta,\alpha} \tau_{\gamma,\beta}^3 \tau_{\gamma,\beta}^4 \quad (3r_T r_V^2) \quad (7725)$$

$$\tau_{\gamma,\alpha}^6 = \sum_{\delta \in A} Z_{\delta,\gamma} \tau_{\delta,\alpha}^5 \quad (2r_T^2 r_V) \quad (7726)$$

$$\tau_{\gamma,\alpha}^4 = \sum_{i \in O} W_{i,\alpha}^1 Y_{i,\gamma}^2 \quad (2r_T r_V N_o) \quad (7739)$$

$$\tau_{\gamma,\alpha}^7 = \sum_{i \in O} W_{i,\alpha}^3 Y_{i,\gamma}^4 \quad (2r_T r_V N_o) \quad (7727)$$

$$\tau_{\gamma,\alpha}^5 = \sum_{\beta \in B} X_{\beta,\alpha} \tau_{\gamma,\beta}^3 \tau_{\gamma,\beta}^4 \quad (3r_T r_V^2) \quad (7740)$$

$$\tau_{\gamma,a}^8 = \sum_{\alpha \in B} W_{a,\alpha}^4 \tau_{\gamma,\alpha}^6 \tau_{\gamma,\alpha}^7 \quad (3r_T r_V N_v) \quad (7728)$$

$$\tau_{\gamma,\alpha}^6 = \sum_{\delta \in A} Z_{\delta,\gamma} \tau_{\delta,\alpha}^5 \quad (2r_T^2 r_V) \quad (7741)$$

$$\tau_{\gamma,\delta}^9 = \sum_{a \in V} Y_{a,\gamma}^1 \tau_{\delta,a}^8 \quad (2r_T^2 N_v) \quad (7729)$$

$$\tau_{\gamma,\alpha}^7 = \sum_{a \in V} W_{a,\alpha}^4 Y_{a,\gamma}^1 \quad (2r_T r_V N_v) \quad (7742)$$

$$\tau_{\gamma,a}^{10} = \sum_{\delta \in A} Y_{a,\delta}^3 \tau_{\gamma,\delta}^9 \quad (2r_T^2 N_v) \quad (7730)$$

$$\tau_{\gamma,\delta,i}^8 = \sum_{\alpha \in B} W_{i,\alpha}^3 \tau_{\delta,\alpha}^6 \tau_{\gamma,\alpha}^7 \quad (3r_T^2 r_V N_o) \quad (7743)$$

$$\tau_{\gamma,\delta,w}^{11} = \sum_{a \in V} {}^2D_{a,w}^3 Y_{a,\delta}^{3,*} \tau_{\gamma,a}^{10} \quad (3r_D r_T^2 N_v) \quad (7731)$$

$$\tau_{\gamma,\delta,\epsilon}^9 = \sum_{i \in O} Z_{\gamma,\delta} Y_{i,\delta}^4 \tau_{\gamma,\epsilon,i}^8 \quad (3r_T^3 N_o) \quad (7744)$$

$$\tau_{\gamma,\delta,w}^{12} = \sum_{\epsilon \in A} Z_{\epsilon,\gamma} \tau_{\epsilon,\delta,w}^{11} \tau_{\epsilon,\delta,w}^2 \quad (3r_D r_T^3) \quad (7732)$$

$$\tau_{\gamma,\delta,i}^{10} = \sum_{\epsilon \in A} Y_{i,\epsilon}^2 \tau_{\epsilon,\gamma,\delta}^9 \quad (2r_T^3 N_o) \quad (7745)$$

$${}^2R_{\gamma,\delta}^z \leftarrow - \sum_{\epsilon \in A} \sum_{w \in D} \frac{1}{2} \tau_{\epsilon,\gamma,w}^0 \tau_{\epsilon,\gamma,w}^1 \tau_{\epsilon,\delta,w}^{12} \quad (3r_D r_T^3) \quad (7733)$$

$$\tau_{\gamma,\delta,w}^{11} = \sum_{\epsilon \in A} \sum_{i \in O} {}^2D_{i,w}^4 Y_{i,\delta}^{4,*} \tau_{\epsilon,\gamma,i}^{10} \tau_{\epsilon,\delta,w}^2 \quad (4r_D r_T^3 N_o) \quad (7746)$$

Raw expression

$${}^2R_{\gamma,\delta}^z \leftarrow - \sum_{\epsilon \in A} \sum_{w \in D} \frac{1}{2} \tau_{\epsilon,\gamma,w}^0 \tau_{\epsilon,\gamma,w}^1 \tau_{\epsilon,\delta,w}^{11} \quad (3r_D r_T^3) \quad (7747)$$

$${}^2R_{\epsilon,\zeta}^z \leftarrow - \sum_{i \in O} \sum_{j \in O} \sum_{k \in O} \sum_{l \in O} \sum_{a \in V} \sum_{b \in V} \sum_{c \in V} \sum_{d \in V} \frac{1}{2} Y_{a,\epsilon}^{1,*} Y_{i,\epsilon}^{2,*} Y_{b,\zeta}^{3,*} Y_{j,\zeta}^{4,*} {}^2D_{a,i,b,j} {}^2T_{c,j,b,l} {}^2T_{d,k,a,i} V_{k,d,l,c} \quad (7734)$$

Raw expression

$${}^2R_{\epsilon,\zeta}^z \leftarrow - \sum_{i \in O} \sum_{j \in O} \sum_{k \in O} \sum_{l \in O} \sum_{a \in V} \sum_{b \in V} \sum_{c \in V} \sum_{d \in V} \frac{1}{2} Y_{a,\epsilon}^{1,*} Y_{i,\epsilon}^{2,*} Y_{b,\zeta}^{3,*} Y_{j,\zeta}^{4,*} {}^2D_{a,i,b,j} {}^2T_{c,k,a,i} {}^2T_{d,l,b,j} V_{k,d,l,c} \quad (7748)$$

Factorized expression

$$\tau_{\gamma,\delta,w}^0 = \sum_{a \in V} {}^2D_{a,w}^1 Y_{a,\gamma}^3 Y_{a,\delta}^{1,*} \quad (3r_D r_T^2 N_v) \quad (7735)$$

Factorized expression

$$\tau_{\gamma,\delta,w}^1 = \sum_{i \in O} {}^2D_{i,w}^2 Y_{i,\gamma}^4 Y_{i,\delta}^{2,*} \quad (3r_D r_T^2 N_o) \quad (7736)$$

$$\tau_{\gamma,\delta,w}^0 = \sum_{a \in V} {}^2D_{a,w}^1 Y_{a,\gamma}^3 Y_{a,\delta}^{1,*} \quad (3r_D r_T^2 N_v) \quad (7749)$$

$$\tau_{\gamma,\delta,w}^2 = \sum_{a \in V} {}^2D_{a,w}^3 Y_{a,\gamma}^3 Y_{a,\delta}^{3,*} \quad (3r_D r_T^2 N_v) \quad (7737)$$

$$\tau_{\gamma,\delta,w}^1 = \sum_{i \in O} {}^2D_{i,w}^2 Y_{i,\gamma}^4 Y_{i,\delta}^{2,*} \quad (3r_D r_T^2 N_o) \quad (7750)$$

$$\tau_{\gamma,\alpha}^3 = \sum_{a \in V} W_{a,\alpha}^2 Y_{a,\gamma}^1 \quad (2r_T r_V N_v) \quad (7738)$$

$$\tau_{\gamma,\delta,w}^2 = \sum_{a \in V} {}^2D_{a,w}^3 Y_{a,\gamma}^3 Y_{a,\delta}^{3,*} \quad (3r_D r_T^2 N_v) \quad (7751)$$



$$\tau^3_{\gamma,\delta,w} = \sum_{i \in O} {}^2D^4_{i,w} Y^4_{i,\gamma} Y^{4,*}_{i,\delta} \quad (3r_D r_T^2 N_o) \quad (7752)$$

$$\tau^1_{\gamma,\delta,w} = \sum_{i \in O} {}^2D^2_{i,w} Y^2_{i,\gamma} Y^{2,*}_{i,\delta} \quad (3r_D r_T^2 N_o) \quad (7765)$$

$$\tau^4_{\gamma,\alpha} = \sum_{a \in V} W^2_{a,\alpha} Y^1_{a,\gamma} \quad (2r_T r_V N_v) \quad (7753)$$

$$\tau^2_{\gamma,\alpha} = \sum_{a \in V} W^2_{a,\alpha} Y^3_{a,\gamma} \quad (2r_T r_V N_v) \quad (7766)$$

$$\tau^5_{\gamma,\alpha,i} = \sum_{\beta \in B} W^1_{i,\beta} X_{\beta,\alpha} \tau^4_{\gamma,\beta} \quad (3r_T r_V^2 N_o) \quad (7754)$$

$$\tau^3_{\gamma,\alpha,i} = \sum_{\beta \in B} W^1_{i,\beta} X_{\beta,\alpha} \tau^2_{\gamma,\beta} \quad (3r_T r_V^2 N_o) \quad (7767)$$

$$\tau^6_{\gamma,\alpha} = \sum_{i \in O} W^3_{i,\alpha} Y^2_{i,\gamma} \quad (2r_T r_V N_o) \quad (7755)$$

$$\tau^4_{\gamma,\alpha} = \sum_{i \in O} W^3_{i,\alpha} Y^4_{i,\gamma} \quad (2r_T r_V N_o) \quad (7768)$$

$$\tau^7_{\gamma,\alpha} = \sum_{a \in V} W^4_{a,\alpha} Y^1_{a,\gamma} \quad (2r_T r_V N_v) \quad (7756)$$

$$\tau^5_{\gamma,\alpha} = \sum_{\delta \in A} \sum_{i \in O} Y^2_{i,\gamma} Z_{\gamma,\delta} \tau^4_{\delta,\alpha} \tau^3_{\delta,\alpha,i} \quad (4r_T^2 r_V N_o) \quad (7769)$$

$$\tau^8_{\gamma,\delta,i} = \sum_{\alpha \in B} \tau^6_{\gamma,\alpha} \tau^7_{\delta,\alpha} \tau^5_{\gamma,\alpha,i} \quad (3r_T^2 r_V N_o) \quad (7757)$$

$$\tau^6_{\gamma,a} = \sum_{\alpha \in B} W^4_{a,\alpha} \tau^5_{\gamma,\alpha} \quad (2r_T r_V N_v) \quad (7770)$$

$$\tau^9_{\gamma,\delta} = \sum_{i \in O} Y^2_{i,\delta} \tau^8_{\gamma,\delta,i} \quad (2r_T^2 N_o) \quad (7758)$$

$$\tau^7_{\gamma,\delta} = \sum_{a \in V} Y^3_{a,\delta} \tau^6_{\gamma,a} \quad (2r_T^2 N_v) \quad (7771)$$

$$\tau^{10}_{\gamma,\delta} = \sum_{\epsilon \in A} Z_{\epsilon,\delta} \tau^9_{\gamma,\epsilon} \quad (2r_T^3) \quad (7759)$$

$$\tau^8_{\gamma,a} = \sum_{\delta \in A} Y^1_{a,\delta} \tau^7_{\delta,\gamma} \quad (2r_T^2 N_v) \quad (7772)$$

$$\tau^{11}_{\gamma,\delta} = \sum_{\epsilon \in A} Z_{\epsilon,\gamma} \tau^{10}_{\epsilon,\delta} \quad (2r_T^3) \quad (7760)$$

$$\tau^9_{\gamma,\delta,w} = \sum_{a \in V} {}^2D^3_{a,w} Y^{3,*}_{a,\delta} \tau^8_{\gamma,a} \quad (3r_D r_T^2 N_v) \quad (7773)$$

$$\tau^{12}_{\gamma,\delta,w} = \sum_{\epsilon \in A} \tau^{11}_{\epsilon,\gamma} \tau^2_{\epsilon,\delta,w} \tau^3_{\epsilon,\delta,w} \quad (3r_D r_T^3) \quad (7761)$$

$$\tau^{10}_{\gamma,\delta,w} = \sum_{i \in O} {}^2D^4_{i,w} Y^4_{i,\gamma} Y^{4,*}_{i,\delta} \quad (3r_D r_T^2 N_o) \quad (7774)$$

$${}^2R^z_{\gamma,\delta} \leftarrow - \sum_{\epsilon \in A} \sum_{w \in D} \frac{1}{2} \tau^0_{\epsilon,\gamma,w} \tau^1_{\epsilon,\gamma,w} \tau^{12}_{\epsilon,\delta,w} \quad (3r_D r_T^3) \quad (7762)$$

$$\tau^{11}_{\gamma,\delta,w} = \sum_{\epsilon \in A} Z_{\gamma,\epsilon} \tau^{10}_{\epsilon,\delta,w} \tau^9_{\epsilon,\delta,w} \quad (3r_D r_T^3) \quad (7775)$$

Raw expression

$${}^2R^z_{\epsilon,\zeta} \leftarrow \sum_{i \in O} \sum_{j \in O} \sum_{k \in O} \sum_{l \in O} \sum_{a \in V} \sum_{b \in V} \sum_{c \in V} \sum_{d \in V} \frac{1}{4} Y^{1,*}_{a,\epsilon} Y^{2,*}_{i,\epsilon} Y^{3,*}_{b,\zeta} Y^{4,*}_{j,\zeta} {}^2D^{a,i,b,j} {}^2T_{a,i,b,k} {}^2T_{c,j,d,l} V_{k,d,l,c} \quad (7763)$$

Factorized expression

$$\tau^0_{\gamma,\delta,w} = \sum_{a \in V} {}^2D^1_{a,w} Y^1_{a,\gamma} Y^{1,*}_{a,\delta} \quad (3r_D r_T^2 N_v) \quad (7764)$$

$${}^2R^z_{\gamma,\delta} \leftarrow \sum_{\epsilon \in A} \sum_{w \in D} \frac{1}{4} \tau^0_{\epsilon,\gamma,w} \tau^1_{\epsilon,\gamma,w} \tau^{11}_{\epsilon,\delta,w} \quad (3r_D r_T^3) \quad (7776)$$

Raw expression

$${}^2R^z_{\epsilon,\zeta} \leftarrow \sum_{i \in O} \sum_{j \in O} \sum_{k \in O} \sum_{l \in O} \sum_{a \in V} \sum_{b \in V} \sum_{c \in V} \sum_{d \in V} \frac{1}{4} Y^{1,*}_{a,\epsilon} Y^{2,*}_{i,\epsilon} Y^{3,*}_{b,\zeta} Y^{4,*}_{j,\zeta} {}^2D^{a,i,b,j} {}^2T_{a,i,b,l} {}^2T_{c,k,d,j} V_{l,c,k,d} \quad (7777)$$

Factorized expression

$$\tau^0_{\gamma,\delta,w} = \sum_{a \in V} {}^2D^1_{a,w} Y^1_{a,\gamma} Y^{1,*}_{a,\delta} \quad (3r_D r_T^2 N_v) \quad (7778)$$

$$\tau^1_{\gamma,\delta,w} = \sum_{i \in O} {}^2D^2_{i,w} Y^2_{i,\gamma} Y^{2,*}_{i,\delta} \quad (3r_D r_T^2 N_o) \quad (7779)$$

$$\tau^2_{\gamma,\delta,w} = \sum_{a \in V} {}^2D^3_{a,w} Y^1_{a,\gamma} Y^{3,*}_{a,\delta} \quad (3r_D r_T^2 N_v) \quad (7780)$$

$$\tau^3_{\gamma,\alpha} = \sum_{a \in V} W^4_{a,\alpha} Y^3_{a,\gamma} \quad (2r_T r_V N_v) \quad (7781)$$

$$\tau^4_{\gamma,\alpha,i} = \sum_{\beta \in B} X_{\alpha,\beta} W^3_{i,\beta} \tau^3_{\gamma,\beta} \quad (3r_T r_V^2 N_o) \quad (7782)$$

$$\tau^5_{\gamma,\alpha} = \sum_{i \in O} W^1_{i,\alpha} Y^4_{i,\gamma} \quad (2r_T r_V N_o) \quad (7783)$$

$$\tau^6_{\gamma,\alpha} = \sum_{a \in V} W^2_{a,\alpha} Y^3_{a,\gamma} \quad (2r_T r_V N_v) \quad (7784)$$

$$\tau^7_{\gamma,\delta,i} = \sum_{\alpha \in B} \tau^5_{\gamma,\alpha} \tau^6_{\delta,\alpha} \tau^4_{\gamma,\alpha,i} \quad (3r_T^2 r_V N_o) \quad (7785)$$

$$\tau^8_{\gamma,\delta,\epsilon} = \sum_{i \in O} Y^2_{i,\gamma} Z_{\gamma,\delta} \tau^7_{\epsilon,\delta,i} \quad (3r_T^3 N_o) \quad (7786)$$

$$\tau^9_{\gamma,\delta,i} = \sum_{\epsilon \in A} Y^4_{i,\epsilon} \tau^8_{\gamma,\epsilon,\delta} \quad (2r_T^3 N_o) \quad (7787)$$

$$\tau^{10}_{\gamma,\delta,w} = \sum_{\epsilon \in A} \sum_{i \in O} {}^2D^4_{i,w} Y^{4,*}_{i,\delta} \tau^2_{\epsilon,\delta,w} \tau^9_{\epsilon,\gamma,i} \quad (4r_D r_T^3 N_o) \quad (7788)$$

$$\tau^{11}_{\gamma,\delta,w} = \sum_{\epsilon \in A} Z_{\gamma,\epsilon} \tau^{10}_{\epsilon,\delta,w} \quad (2r_D r_T^3) \quad (7789)$$

$${}^2R^z_{\gamma,\delta} \leftarrow \sum_{\epsilon \in A} \sum_{w \in D} \frac{1}{4} \tau^0_{\epsilon,\gamma,w} \tau^1_{\epsilon,\gamma,w} \tau^{11}_{\epsilon,\delta,w} \quad (3r_D r_T^3) \quad (7790)$$

Raw expression

$${}^2R^z_{\epsilon,\zeta} \leftarrow \sum_{i \in O} \sum_{j \in O} \sum_{k \in O} \sum_{l \in O} \sum_{a \in V} \sum_{b \in V} \sum_{c \in V} \sum_{d \in V} \frac{1}{4} Y^{1,*}_{a,\epsilon} Y^{2,*}_{i,\epsilon} Y^{3,*}_{b,\zeta} Y^{4,*}_{j,\zeta} {}^2D^{a,i,b,j} {}^2T_{a,i,c,j} {}^2T_{b,k,d,l} V_{k,d,l,c} \quad (7791)$$

Factorized expression

$$\tau^0_{\gamma,\delta,w} = \sum_{a \in V} {}^2D^1_{a,w} Y^1_{a,\gamma} Y^{1,*}_{a,\delta} \quad (3r_D r_T^2 N_v) \quad (7792)$$

$$\tau^1_{\gamma,\alpha} = \sum_{i \in O} W^1_{i,\alpha} Y^2_{i,\gamma} \quad (2r_T r_V N_o) \quad (7793)$$

$$\tau^2_{\gamma,\alpha} = \sum_{a \in V} W^2_{a,\alpha} Y^3_{a,\gamma} \quad (2r_T r_V N_v) \quad (7794)$$

$$\tau^3_{\gamma,\alpha,i} = \sum_{\delta \in A} Z_{\gamma,\delta} Y^4_{i,\delta} \tau^2_{\delta,\alpha} \quad (3r_T^2 r_V N_o) \quad (7795)$$

$$\tau^4_{\gamma,\alpha,w} = \sum_{\delta \in A} \sum_{i \in O} {}^2D^2_{i,w} Y^{2,*}_{i,\gamma} \tau^1_{\delta,\alpha} \tau^0_{\delta,\gamma,w} \tau^3_{\delta,\alpha,i} \quad (5r_D r_T^2 r_V N_o) \quad (7796)$$

$$\tau^5_{\gamma,\alpha,w} = \sum_{\beta \in B} X_{\beta,\alpha} \tau^4_{\gamma,\beta,w} \quad (2r_D r_T r_V^2) \quad (7797)$$

$$\tau^6_{\gamma,\delta,w} = \sum_{a \in V} {}^2D^3_{a,w} Y^1_{a,\gamma} Y^{3,*}_{a,\delta} \quad (3r_D r_T^2 N_v) \quad (7798)$$

$$\tau^7_{\gamma,\alpha} = \sum_{i \in O} W^3_{i,\alpha} Y^2_{i,\gamma} \quad (2r_T r_V N_o) \quad (7799)$$

$$\tau^8_{\gamma,\alpha} = \sum_{a \in V} W^4_{a,\alpha} Y^3_{a,\gamma} \quad (2r_T r_V N_v) \quad (7800)$$

$$\tau^9_{\gamma,\alpha,i} = \sum_{\delta \in A} Z_{\gamma,\delta} Y^4_{i,\delta} \tau^8_{\delta,\alpha} \quad (3r_T^2 r_V N_o) \quad (7801)$$

$$\tau^{10}_{\gamma,\alpha,w} = \sum_{\delta \in A} \sum_{i \in O} {}^2D^4_{i,w} Y^{4,*}_{i,\gamma} \tau^7_{\delta,\alpha} \tau^6_{\delta,\gamma,w} \tau^9_{\delta,\alpha,i} \quad (5r_D r_T^2 r_V N_o) \quad (7802)$$

$${}^2R^z_{\gamma,\delta} \leftarrow \sum_{\alpha \in B} \sum_{w \in D} \frac{1}{4} \tau^{10}_{\delta,\alpha,w} \tau^5_{\gamma,\alpha,w} \quad (2r_D r_T^2 r_V) \quad (7803)$$

Raw expression

$${}^2R^z_{\epsilon,\zeta} \leftarrow \sum_{i \in O} \sum_{j \in O} \sum_{k \in O} \sum_{l \in O} \sum_{a \in V} \sum_{b \in V} \sum_{c \in V} \sum_{d \in V} \frac{1}{4} Y^{1,*}_{a,\epsilon} Y^{2,*}_{i,\epsilon} Y^{3,*}_{b,\zeta} Y^{4,*}_{j,\zeta} {}^2D^{a,i,b,j} {}^2T_{a,i,c,j} {}^2T_{d,k,b,l} V_{k,c,l,d} \quad (7804)$$

Factorized expression

$$\tau_{\gamma,\delta,w}^0 = \sum_{a \in V} {}^2D_{a,w}^1 Y_{a,\gamma}^1 Y_{a,\delta}^{1,*} \quad (3r_D r_T^2 N_v) \quad (7805)$$

$$\tau_{\gamma,\alpha}^1 = \sum_{a \in V} W_{a,\alpha}^2 Y_{a,\gamma}^3 \quad (2r_T r_V N_v) \quad (7806)$$

$$\tau_{\gamma,\alpha,i}^2 = \sum_{\beta \in B} W_{i,\beta}^1 X_{\beta,\alpha} \tau_{\gamma,\beta}^1 \quad (3r_T r_V^2 N_o) \quad (7807)$$

$$\tau_{\gamma,\delta,\alpha}^3 = \sum_{i \in O} Y_{i,\gamma}^2 \tau_{\delta,\alpha,i}^2 \quad (2r_T^2 r_V N_o) \quad (7808)$$

$$\tau_{\gamma,\delta,w}^4 = \sum_{a \in V} {}^2D_{a,w}^3 Y_{a,\gamma}^1 Y_{a,\delta}^{3,*} \quad (3r_D r_T^2 N_v) \quad (7809)$$

$$\tau_{\gamma,\delta,w,i}^5 = \sum_{\epsilon \in A} Y_{i,\epsilon}^2 Z_{\epsilon,\gamma} \tau_{\epsilon,\delta,w}^4 \quad (3r_D r_T^3 N_o) \quad (7810)$$

$$\tau_{\gamma,\delta,\alpha,w}^6 = \sum_{i \in O} W_{i,\alpha}^3 \tau_{\gamma,\delta,w,i}^5 \quad (2r_D r_T^2 r_V N_o) \quad (7811)$$

$$\tau_{\gamma,\alpha}^7 = \sum_{a \in V} W_{a,\alpha}^4 Y_{a,\gamma}^3 \quad (2r_T r_V N_v) \quad (7812)$$

$$\tau_{\gamma,\alpha,i}^8 = \sum_{\delta \in A} Z_{\gamma,\delta} Y_{i,\delta}^4 \tau_{\delta,\alpha}^7 \quad (3r_T^2 r_V N_o) \quad (7813)$$

$$\tau_{\gamma,\delta,\alpha,w}^9 = \sum_{i \in O} {}^2D_{i,w}^4 Y_{i,\delta}^{4,*} \tau_{\gamma,\alpha,i}^8 \quad (3r_D r_T^2 r_V N_o) \quad (7814)$$

$$\tau_{\gamma,\delta,\epsilon,w}^{10} = \sum_{\alpha \in B} \tau_{\gamma,\delta,\alpha}^3 \tau_{\delta,\epsilon,\alpha,w}^6 \tau_{\gamma,\epsilon,\alpha,w}^9 \quad (3r_D r_T^3 r_V) \quad (7815)$$

$$\tau_{\gamma,\delta,w,i}^{11} = \sum_{\epsilon \in A} {}^2D_{i,w}^2 Y_{i,\epsilon}^4 \tau_{\gamma,\epsilon,\delta,w}^{10} \quad (3r_D r_T^3 N_o) \quad (7816)$$

$$\tau_{\gamma,\delta,i}^{12} = \sum_{\epsilon \in A} \sum_{w \in D} \tau_{\epsilon,\gamma,w}^0 \tau_{\epsilon,\delta,w,i}^{11} \quad (2r_D r_T^3 N_o) \quad (7817)$$

$${}^2R_{\gamma,\delta}^z \leftarrow \sum_{i \in O} \frac{1}{4} Y_{i,\gamma}^{2,*} \tau_{\gamma,\delta,i}^{12} \quad (2r_T^2 N_o) \quad (7818)$$

Raw expression

$${}^2R_{\epsilon,\zeta}^z \leftarrow \sum_{i \in O} \sum_{j \in O} \sum_{k \in O} \sum_{l \in O} \sum_{a \in V} \sum_{b \in V} \sum_{c \in V} \sum_{d \in V} \frac{1}{4} Y_{a,\epsilon}^{1,*} Y_{i,\epsilon}^{2,*} Y_{b,\zeta}^{3,*} Y_{j,\zeta}^{4,*} {}^2D_{a,i,b,j} {}^2T_{a,i,c,k} {}^2T_{d,j,b,l} V_{k,d,l,c} \quad (7819)$$

Factorized expression

$$\tau_{\gamma,\delta,w}^0 = \sum_{a \in V} {}^2D_{a,w}^1 Y_{a,\gamma}^1 Y_{a,\delta}^{1,*} \quad (3r_D r_T^2 N_v) \quad (7820)$$

$$\tau_{\gamma,\delta,w}^1 = \sum_{i \in O} {}^2D_{i,w}^2 Y_{i,\gamma}^2 Y_{i,\delta}^{2,*} \quad (3r_D r_T^2 N_o) \quad (7821)$$

$$\tau_{\gamma,\delta,w}^2 = \sum_{a \in V} {}^2D_{a,w}^3 Y_{a,\gamma}^3 Y_{a,\delta}^{3,*} \quad (3r_D r_T^2 N_v) \quad (7822)$$

$$\tau_{\gamma,\alpha}^3 = \sum_{a \in V} W_{a,\alpha}^4 Y_{a,\gamma}^3 \quad (2r_T r_V N_v) \quad (7823)$$

$$\tau_{\gamma,\alpha,i}^4 = \sum_{\beta \in B} X_{\alpha,\beta} W_{i,\beta}^3 \tau_{\gamma,\beta}^3 \quad (3r_T r_V^2 N_o) \quad (7824)$$

$$\tau_{\gamma,\alpha}^5 = \sum_{i \in O} W_{i,\alpha}^1 Y_{i,\gamma}^4 \quad (2r_T r_V N_o) \quad (7825)$$

$$\tau_{\gamma,\alpha}^6 = \sum_{a \in V} W_{a,\alpha}^2 Y_{a,\gamma}^1 \quad (2r_T r_V N_v) \quad (7826)$$

$$\tau_{\gamma,\delta,i}^7 = \sum_{\alpha \in B} \tau_{\delta,\alpha}^5 \tau_{\gamma,\alpha}^6 \tau_{\delta,\alpha,i}^4 \quad (3r_T^2 r_V N_o) \quad (7827)$$

$$\tau_{\gamma,\delta,\epsilon}^8 = \sum_{i \in O} Z_{\gamma,\delta} Y_{i,\delta}^4 \tau_{\gamma,\epsilon,i}^7 \quad (3r_T^3 N_o) \quad (7828)$$

$$\tau_{\gamma,\delta,i}^9 = \sum_{\epsilon \in A} Y_{i,\epsilon}^2 \tau_{\epsilon,\gamma,\delta}^8 \quad (2r_T^3 N_o) \quad (7829)$$

$$\tau_{\gamma,\delta,w}^{10} = \sum_{\epsilon \in A} \sum_{i \in O} {}^2D_{i,w}^4 Y_{i,\delta}^{4,*} \tau_{\epsilon,\delta,w}^2 \tau_{\epsilon,\gamma,i}^9 \quad (4r_D r_T^3 N_o) \quad (7830)$$

$$\tau_{\gamma,\delta,w}^{11} = \sum_{\epsilon \in A} Z_{\gamma,\epsilon} \tau_{\epsilon,\delta,w}^{10} \quad (2r_D r_T^3) \quad (7831)$$

$${}^2R^z_{\gamma,\delta} \leftarrow \sum_{\epsilon \in A} \sum_{w \in D} \frac{1}{4} \tau^0_{\epsilon,\gamma,w} \tau^1_{\epsilon,\gamma,w} \tau^{11}_{\epsilon,\delta,w} \quad (3r_D r_T^3) \quad (7832)$$

Raw expression

$${}^2R^z_{\epsilon,\zeta} \leftarrow \sum_{i \in O} \sum_{j \in O} \sum_{k \in O} \sum_{l \in O} \sum_{a \in V} \sum_{b \in V} \sum_{c \in V} \sum_{d \in V} \frac{1}{4} Y^{1,*}_{a,\epsilon} Y^{2,*}_{i,\epsilon} Y^{3,*}_{b,\zeta} Y^{4,*}_{j,\zeta} {}^2D^{a,i,b,j} {}^2T_{a,i,c,l} {}^2T_{b,k,d,j} V_{l,d,k,c} \quad (7833)$$

Factorized expression

$$\tau^0_{\gamma,\delta,w} = \sum_{a \in V} {}^2D^1_{a,w} Y^1_{a,\gamma} Y^{1,*}_{a,\delta} \quad (3r_D r_T^2 N_v) \quad (7834)$$

$$\tau^1_{\gamma,\delta,w} = \sum_{i \in O} {}^2D^2_{i,w} Y^2_{i,\gamma} Y^{2,*}_{i,\delta} \quad (3r_D r_T^2 N_o) \quad (7835)$$

$$\tau^2_{\gamma,\delta,w} = \sum_{a \in V} {}^2D^3_{a,w} Y^3_{a,\gamma} Y^{3,*}_{a,\delta} \quad (3r_D r_T^2 N_v) \quad (7836)$$

$$\tau^3_{\gamma,\alpha} = \sum_{a \in V} W^2_{a,\alpha} Y^1_{a,\gamma} \quad (2r_T r_V N_v) \quad (7837)$$

$$\tau^4_{\gamma,\alpha,i} = \sum_{\beta \in B} W^1_{i,\beta} X_{\beta,\alpha} \tau^3_{\gamma,\beta} \quad (3r_T r_V^2 N_o) \quad (7838)$$

$$\tau^5_{\gamma,\alpha} = \sum_{i \in O} W^3_{i,\alpha} Y^2_{i,\gamma} \quad (2r_T r_V N_o) \quad (7839)$$

$$\tau^6_{\gamma,\alpha} = \sum_{a \in V} W^4_{a,\alpha} Y^3_{a,\gamma} \quad (2r_T r_V N_v) \quad (7840)$$

$$\tau^7_{\gamma,\delta,i} = \sum_{\alpha \in B} \tau^5_{\gamma,\alpha} \tau^6_{\delta,\alpha} \tau^4_{\gamma,\alpha,i} \quad (3r_T^2 r_V N_o) \quad (7841)$$

$$\tau^8_{\gamma,i} = \sum_{\delta \in A} Z_{\delta,\gamma} \tau^7_{\delta,\gamma,i} \quad (2r_T^2 N_o) \quad (7842)$$

$$\tau^9_{i,j} = \sum_{\gamma \in A} Y^4_{j,\gamma} \tau^8_{\gamma,i} \quad (2r_T N_o^2) \quad (7843)$$

$$\tau^{10}_{\gamma,i} = \sum_{j \in O} Y^4_{j,\gamma} \tau^9_{j,i} \quad (2r_T N_o^2) \quad (7844)$$

$$\tau^{11}_{\gamma,\delta,w} = \sum_{i \in O} {}^2D^4_{i,w} Y^{4,*}_{i,\delta} \tau^{10}_{\gamma,i} \quad (3r_D r_T^2 N_o) \quad (7845)$$

$$\tau^{12}_{\gamma,\delta,w} = \sum_{\epsilon \in A} Z_{\gamma,\epsilon} \tau^{11}_{\epsilon,\delta,w} \tau^2_{\epsilon,\delta,w} \quad (3r_D r_T^3) \quad (7846)$$

$${}^2R^z_{\gamma,\delta} \leftarrow \sum_{\epsilon \in A} \sum_{w \in D} \frac{1}{4} \tau^0_{\epsilon,\gamma,w} \tau^1_{\epsilon,\gamma,w} \tau^{12}_{\epsilon,\delta,w} \quad (3r_D r_T^3) \quad (7847)$$

Raw expression

$${}^2R^z_{\epsilon,\zeta} \leftarrow \sum_{i \in O} \sum_{j \in O} \sum_{k \in O} \sum_{l \in O} \sum_{a \in V} \sum_{b \in V} \sum_{c \in V} \sum_{d \in V} \frac{1}{4} Y^{1,*}_{a,\epsilon} Y^{2,*}_{i,\epsilon} Y^{3,*}_{b,\zeta} Y^{4,*}_{j,\zeta} {}^2D^{a,i,b,j} {}^2T_{a,k,b,j} {}^2T_{c,i,d,l} V_{k,d,l,c} \quad (7848)$$

Factorized expression

$$\tau^0_{\gamma,\alpha} = \sum_{a \in V} W^2_{a,\alpha} Y^1_{a,\gamma} \quad (2r_T r_V N_v) \quad (7849)$$

$$\tau^1_{\gamma,\alpha,i} = \sum_{\beta \in B} W^1_{i,\beta} X_{\beta,\alpha} \tau^0_{\gamma,\beta} \quad (3r_T r_V^2 N_o) \quad (7850)$$

$$\tau^2_{\gamma,\alpha} = \sum_{i \in O} W^3_{i,\alpha} Y^2_{i,\gamma} \quad (2r_T r_V N_o) \quad (7851)$$

$$\tau^3_{\gamma,\alpha} = \sum_{a \in V} W^4_{a,\alpha} Y^3_{a,\gamma} \quad (2r_T r_V N_v) \quad (7852)$$

$$\tau^4_{\gamma,\delta,i} = \sum_{\alpha \in B} \tau^2_{\gamma,\alpha} \tau^3_{\delta,\alpha} \tau^1_{\gamma,\alpha,i} \quad (3r_T^2 r_V N_o) \quad (7853)$$

$$\tau^5_{\gamma,i} = \sum_{\delta \in A} Z_{\delta,\gamma} \tau^4_{\delta,\gamma,i} \quad (2r_T^2 N_o) \quad (7854)$$

$$\tau^6_{i,j} = \sum_{\gamma \in A} Y^4_{j,\gamma} \tau^5_{\gamma,i} \quad (2r_T N_o^2) \quad (7855)$$

$$\tau^7_{\gamma,i} = \sum_{j \in O} Y^2_{j,\gamma} \tau^6_{j,i} \quad (2r_T N_o^2) \quad (7856)$$

$$\tau^8_{\gamma,\delta,w} = \sum_{i \in O} {}^2D^2_{i,w} Y^{2,*}_{i,\delta} \tau^7_{\gamma,i} \quad (3r_D r_T^2 N_o) \quad (7857)$$

$$\tau^9_{\gamma,\delta,w} = \sum_{a \in V} {}^2D^1_{a,w} Y^1_{a,\gamma} Y^{1,*}_{a,\delta} \quad (3r_D r_T^2 N_v) \quad (7858)$$

$$\tau^7_{\gamma,\delta,i} = \sum_{\epsilon \in A} Y^4_{i,\epsilon} \tau^6_{\gamma,\delta,\epsilon} \quad (2r_T^3 N_o) \quad (7871)$$

$$\tau^{10}_{\gamma,\delta,w} = \sum_{a \in V} {}^2D^3_{a,w} Y^3_{a,\gamma} Y^{3,*}_{a,\delta} \quad (3r_D r_T^2 N_v) \quad (7859)$$

$$\tau^8_{\gamma,\delta,w} = \sum_{\epsilon \in A} \sum_{i \in O} {}^2D^2_{i,w} Y^{2,*}_{i,\delta} \tau^0_{\epsilon,\delta,w} \tau^7_{\gamma,\epsilon,i} \quad (4r_D r_T^3 N_o) \quad (7872)$$

$$\tau^{11}_{\gamma,\delta,w} = \sum_{i \in O} {}^2D^4_{i,w} Y^4_{i,\gamma} Y^{4,*}_{i,\delta} \quad (3r_D r_T^2 N_o) \quad (7860)$$

$$\tau^9_{\gamma,\delta,w} = \sum_{\epsilon \in A} Z_{\epsilon,\gamma} \tau^8_{\epsilon,\delta,w} \quad (2r_D r_T^3) \quad (7873)$$

$$\tau^{12}_{\gamma,\delta,w} = \sum_{\epsilon \in A} Z_{\gamma,\epsilon} \tau^{10}_{\epsilon,\delta,w} \tau^{11}_{\epsilon,\delta,w} \quad (3r_D r_T^3) \quad (7861)$$

$$\tau^{10}_{\gamma,\delta,w} = \sum_{a \in V} {}^2D^3_{a,w} Y^3_{a,\gamma} Y^{3,*}_{a,\delta} \quad (3r_D r_T^2 N_v) \quad (7874)$$

$${}^2R^z_{\gamma,\delta} \leftarrow \sum_{\epsilon \in A} \sum_{w \in D} \frac{1}{4} \tau^{12}_{\epsilon,\delta,w} \tau^8_{\epsilon,\gamma,w} \tau^9_{\epsilon,\gamma,w} \quad (3r_D r_T^3) \quad (7862)$$

$$\tau^{11}_{\gamma,\delta,w} = \sum_{i \in O} {}^2D^4_{i,w} Y^4_{i,\gamma} Y^{4,*}_{i,\delta} \quad (3r_D r_T^2 N_o) \quad (7875)$$

Raw expression

$${}^2R^z_{\epsilon,\zeta} \leftarrow \sum_{i \in O} \sum_{j \in O} \sum_{k \in O} \sum_{l \in O} \sum_{a \in V} \sum_{b \in V} \sum_{c \in V} \sum_{d \in V} \frac{1}{4} Y^{1,*}_{a,\epsilon} Y^{2,*}_{i,\epsilon} Y^{3,*}_{b,\zeta} Y^{4,*}_{j,\zeta} {}^2D^{a,i,b,j} {}^2T_{a,k,b,j} {}^2T_{c,l,d,i} V_{k,c,l,d} \quad (7863)$$

$${}^2R^z_{\gamma,\delta} \leftarrow \sum_{\epsilon \in A} \sum_{w \in D} \frac{1}{4} \tau^{10}_{\epsilon,\delta,w} \tau^{11}_{\epsilon,\delta,w} \tau^9_{\epsilon,\gamma,w} \quad (3r_D r_T^3) \quad (7876)$$

Raw expression

$${}^2R^z_{\epsilon,\zeta} \leftarrow \sum_{i \in O} \sum_{j \in O} \sum_{k \in O} \sum_{l \in O} \sum_{a \in V} \sum_{b \in V} \sum_{c \in V} \sum_{d \in V} \frac{1}{4} Y^{1,*}_{a,\epsilon} Y^{2,*}_{i,\epsilon} Y^{3,*}_{b,\zeta} Y^{4,*}_{j,\zeta} {}^2D^{a,i,b,j} {}^2T_{a,k,b,l} {}^2T_{c,i,d,j} V_{k,c,l,d} \quad (7877)$$

Factorized expression

$$\tau^0_{\gamma,\delta,w} = \sum_{a \in V} {}^2D^1_{a,w} Y^1_{a,\gamma} Y^{1,*}_{a,\delta} \quad (3r_D r_T^2 N_v) \quad (7864)$$

Factorized expression

$$\tau^0_{\gamma,\delta,w} = \sum_{a \in V} {}^2D^1_{a,w} Y^1_{a,\gamma} Y^{1,*}_{a,\delta} \quad (3r_D r_T^2 N_v) \quad (7878)$$

$$\tau^1_{\gamma,\alpha} = \sum_{a \in V} W^2_{a,\alpha} Y^1_{a,\gamma} \quad (2r_T r_V N_v) \quad (7865)$$

$$\tau^2_{\gamma,\alpha,i} = \sum_{\beta \in B} W^1_{i,\beta} X_{\beta,\alpha} \tau^1_{\gamma,\beta} \quad (3r_T r_V^2 N_o) \quad (7866)$$

$$\tau^1_{\gamma,\delta,w} = \sum_{i \in O} {}^2D^2_{i,w} Y^2_{i,\gamma} Y^{2,*}_{i,\delta} \quad (3r_D r_T^2 N_o) \quad (7879)$$

$$\tau^3_{\gamma,\alpha} = \sum_{i \in O} W^3_{i,\alpha} Y^2_{i,\gamma} \quad (2r_T r_V N_o) \quad (7867)$$

$$\tau^2_{\gamma,\delta,w} = \sum_{a \in V} {}^2D^3_{a,w} Y^3_{a,\gamma} Y^{3,*}_{a,\delta} \quad (3r_D r_T^2 N_v) \quad (7880)$$

$$\tau^4_{\gamma,\alpha} = \sum_{a \in V} W^4_{a,\alpha} Y^3_{a,\gamma} \quad (2r_T r_V N_v) \quad (7868)$$

$$\tau^3_{\gamma,\alpha} = \sum_{a \in V} W^2_{a,\alpha} Y^3_{a,\gamma} \quad (2r_T r_V N_v) \quad (7881)$$

$$\tau^5_{\gamma,\delta,i} = \sum_{\alpha \in B} \tau^3_{\gamma,\alpha} \tau^4_{\delta,\alpha} \tau^2_{\gamma,\alpha,i} \quad (3r_T^2 r_V N_o) \quad (7869)$$

$$\tau^4_{\gamma,\alpha,i} = \sum_{\beta \in B} W^1_{i,\beta} X_{\beta,\alpha} \tau^3_{\gamma,\beta} \quad (3r_T r_V^2 N_o) \quad (7882)$$

$$\tau^6_{\gamma,\delta,\epsilon} = \sum_{i \in O} Y^2_{i,\delta} Z_{\delta,\epsilon} \tau^5_{\gamma,\epsilon,i} \quad (3r_T^3 N_o) \quad (7870)$$

$$\tau^5_{\gamma,\alpha} = \sum_{i \in O} W^3_{i,\alpha} Y^4_{i,\gamma} \quad (2r_T r_V N_o) \quad (7883)$$

$$\tau_{\gamma,\alpha}^6 = \sum_{a \in V} W_{a,\alpha}^4 Y_{a,\gamma}^1 \quad (2r_T r_V N_v) \quad (7884)$$

$$\tau_{\gamma,\alpha}^4 = \sum_{i \in O} W_{i,\alpha}^1 Y_{i,\gamma}^2 \quad (2r_T r_V N_o) \quad (7897)$$

$$\tau_{\gamma,\delta,i}^7 = \sum_{\alpha \in B} \tau_{\delta,\alpha}^5 \tau_{\gamma,\alpha}^6 \tau_{\delta,\alpha,i}^4 \quad (3r_T^2 r_V N_o) \quad (7885)$$

$$\tau_{\gamma,\alpha}^5 = \sum_{\delta \in A} \sum_{i \in O} Z_{\delta,\gamma} Y_{i,\gamma}^4 \tau_{\delta,\alpha}^4 \tau_{\delta,\alpha,i}^3 \quad (4r_T^2 r_V N_o) \quad (7898)$$

$$\tau_{\gamma,i}^8 = \sum_{\delta \in A} Z_{\gamma,\delta} \tau_{\gamma,\delta,i}^7 \quad (2r_T^2 N_o) \quad (7886)$$

$$\tau_{\gamma,a}^6 = \sum_{\alpha \in B} W_{a,\alpha}^2 \tau_{\gamma,\alpha}^5 \quad (2r_T r_V N_v) \quad (7899)$$

$$\tau_{i,j}^9 = \sum_{\gamma \in A} Y_{j,\gamma}^2 \tau_{\gamma,i}^8 \quad (2r_T N_o^2) \quad (7887)$$

$$\tau_{a,b}^7 = \sum_{\gamma \in A} Y_{b,\gamma}^3 \tau_{\gamma,a}^6 \quad (2r_T N_v^2) \quad (7900)$$

$$\tau_{\gamma,i}^{10} = \sum_{j \in O} Y_{j,\gamma}^4 \tau_{j,i}^9 \quad (2r_T N_o^2) \quad (7888)$$

$$\tau_{\gamma,a}^8 = \sum_{b \in V} Y_{b,\gamma}^3 \tau_{b,a}^7 \quad (2r_T N_v^2) \quad (7901)$$

$$\tau_{\gamma,\delta,w}^{11} = \sum_{i \in O} {}^2D_{i,w}^4 Y_{i,\delta}^{4,*} \tau_{\gamma,i}^{10} \quad (3r_D r_T^2 N_o) \quad (7889)$$

$$\tau_{\gamma,\delta,w}^9 = \sum_{a \in V} {}^2D_{a,w}^3 Y_{a,\delta}^{3,*} \tau_{\gamma,a}^8 \quad (3r_D r_T^2 N_v) \quad (7902)$$

$$\tau_{\gamma,\delta,w}^{12} = \sum_{\epsilon \in A} Z_{\gamma,\epsilon} \tau_{\epsilon,\delta,w}^{11} \tau_{\epsilon,\delta,w}^2 \quad (3r_D r_T^3) \quad (7890)$$

$$\tau_{\gamma,\delta,w}^{10} = \sum_{i \in O} {}^2D_{i,w}^4 Y_{i,\gamma}^4 Y_{i,\delta}^{4,*} \quad (3r_D r_T^2 N_o) \quad (7903)$$

$${}^2R_{\gamma,\delta}^z \leftarrow \sum_{\epsilon \in A} \sum_{w \in D} \frac{1}{4} \tau_{\epsilon,\gamma,w}^0 \tau_{\epsilon,\gamma,w}^1 \tau_{\epsilon,\delta,w}^{12} \quad (3r_D r_T^3) \quad (7891)$$

$$\tau_{\gamma,\delta,w}^{11} = \sum_{\epsilon \in A} Z_{\gamma,\epsilon} \tau_{\epsilon,\delta,w}^{10} \tau_{\epsilon,\delta,w}^9 \quad (3r_D r_T^3) \quad (7904)$$

Raw expression

$${}^2R_{\epsilon,\zeta}^z \leftarrow \sum_{i \in O} \sum_{j \in O} \sum_{k \in O} \sum_{l \in O} \sum_{a \in V} \sum_{b \in V} \sum_{c \in V} \sum_{d \in V} \frac{1}{4} Y_{a,\epsilon}^{1,*} Y_{i,\epsilon}^{2,*} Y_{b,\zeta}^{3,*} Y_{j,\zeta}^{4,*} {}^2D_{a,i,b,j} {}^2T_{a,k,b,l} {}^2T_{c,j,d,i} V_{k,d,l,c} \quad (7892)$$

$${}^2R_{\gamma,\delta}^z \leftarrow \sum_{\epsilon \in A} \sum_{w \in D} \frac{1}{4} \tau_{\epsilon,\gamma,w}^0 \tau_{\epsilon,\gamma,w}^1 \tau_{\epsilon,\delta,w}^{11} \quad (3r_D r_T^3) \quad (7905)$$

Raw expression

$${}^2R_{\epsilon,\zeta}^z \leftarrow \sum_{i \in O} \sum_{j \in O} \sum_{k \in O} \sum_{l \in O} \sum_{a \in V} \sum_{b \in V} \sum_{c \in V} \sum_{d \in V} \frac{1}{4} Y_{a,\epsilon}^{1,*} Y_{i,\epsilon}^{2,*} Y_{b,\zeta}^{3,*} Y_{j,\zeta}^{4,*} {}^2D_{a,i,b,j} {}^2T_{a,k,c,i} {}^2T_{b,l,d,j} V_{k,c,l,d} \quad (7906)$$

Factorized expression

$$\tau_{\gamma,\delta,w}^0 = \sum_{a \in V} {}^2D_{a,w}^1 Y_{a,\gamma}^1 Y_{a,\delta}^{1,*} \quad (3r_D r_T^2 N_v) \quad (7893)$$

Factorized expression

$$\tau_{\gamma,\delta,w}^1 = \sum_{i \in O} {}^2D_{i,w}^2 Y_{i,\gamma}^2 Y_{i,\delta}^{2,*} \quad (3r_D r_T^2 N_o) \quad (7894)$$

$$\tau_{\gamma,\alpha}^0 = \sum_{a \in V} W_{a,\alpha}^2 Y_{a,\gamma}^3 \quad (2r_T r_V N_v) \quad (7907)$$

$$\tau_{\gamma,\alpha}^2 = \sum_{a \in V} W_{a,\alpha}^4 Y_{a,\gamma}^1 \quad (2r_T r_V N_v) \quad (7895)$$

$$\tau_{\gamma,\alpha,i}^1 = \sum_{\beta \in B} W_{i,\beta}^1 X_{\beta,\alpha} \tau_{\gamma,\beta}^0 \quad (3r_T r_V^2 N_o) \quad (7908)$$

$$\tau_{\gamma,\alpha,i}^3 = \sum_{\beta \in B} X_{\alpha,\beta} W_{i,\beta}^3 \tau_{\gamma,\beta}^2 \quad (3r_T r_V^2 N_o) \quad (7896)$$

$$\tau_{\gamma,\alpha}^2 = \sum_{i \in O} W_{i,\alpha}^3 Y_{i,\gamma}^4 \quad (2r_T r_V N_o) \quad (7909)$$

$$\tau^3_{\gamma,\alpha} = \sum_{\delta \in A} \sum_{i \in O} Y^2_{i,\gamma} Z_{\gamma,\delta} \tau^2_{\delta,\alpha} \tau^1_{\delta,\alpha,i} \quad (4r_T^2 r_V N_o) \quad (7910)$$

$$\tau^4_{\gamma,a} = \sum_{\alpha \in B} W^4_{a,\alpha} \tau^3_{\gamma,\alpha} \quad (2r_T r_V N_v) \quad (7911)$$

$$\tau^5_{\gamma,\delta} = \sum_{a \in V} Y^3_{a,\delta} \tau^4_{\gamma,a} \quad (2r_T^2 N_v) \quad (7912)$$

$$\tau^6_{\gamma,a} = \sum_{\delta \in A} Y^1_{a,\delta} \tau^5_{\delta,\gamma} \quad (2r_T^2 N_v) \quad (7913)$$

$$\tau^7_{\gamma,\delta,w} = \sum_{a \in V} {}^2D^1_{a,w} Y^{1,*}_{a,\delta} \tau^6_{\gamma,a} \quad (3r_D r_T^2 N_v) \quad (7914)$$

$$\tau^8_{\gamma,\delta,w} = \sum_{i \in O} {}^2D^2_{i,w} Y^4_{i,\gamma} Y^{2,*}_{i,\delta} \quad (3r_D r_T^2 N_o) \quad (7915)$$

$$\tau^9_{\gamma,\delta,w} = \sum_{a \in V} {}^2D^3_{a,w} Y^1_{a,\gamma} Y^{3,*}_{a,\delta} \quad (3r_D r_T^2 N_v) \quad (7916)$$

$$\tau^{10}_{\gamma,\delta,w} = \sum_{i \in O} {}^2D^4_{i,w} Y^2_{i,\gamma} Y^{4,*}_{i,\delta} \quad (3r_D r_T^2 N_o) \quad (7917)$$

$$\tau^{11}_{\gamma,\delta,w} = \sum_{\epsilon \in A} Z_{\epsilon,\gamma} \tau^{10}_{\epsilon,\delta,w} \tau^9_{\epsilon,\delta,w} \quad (3r_D r_T^3) \quad (7918)$$

$${}^2R^z_{\gamma,\delta} \leftarrow \sum_{\epsilon \in A} \sum_{w \in D} \frac{1}{4} \tau^{11}_{\epsilon,\delta,w} \tau^7_{\epsilon,\gamma,w} \tau^8_{\epsilon,\gamma,w} \quad (3r_D r_T^3) \quad (7919)$$

Raw expression

$${}^2R^z_{\epsilon,\zeta} \leftarrow \sum_{i \in O} \sum_{j \in O} \sum_{k \in O} \sum_{l \in O} \sum_{a \in V} \sum_{b \in V} \sum_{c \in V} \sum_{d \in V} \frac{1}{4} Y^{1,*}_{a,\epsilon} Y^{2,*}_{i,\epsilon} Y^{3,*}_{b,\zeta} Y^{4,*}_{j,\zeta} {}^2D^{a,i,b,j} {}^2T_{a,k,c,i} {}^2T_{d,l,b,j} V_{k,d,l,c} \quad (7920)$$

Factorized expression

$$\tau^0_{\gamma,\delta,w} = \sum_{a \in V} {}^2D^1_{a,w} Y^1_{a,\gamma} Y^{1,*}_{a,\delta} \quad (3r_D r_T^2 N_v) \quad (7921)$$

$$\tau^1_{\gamma,\alpha} = \sum_{a \in V} W^2_{a,\alpha} Y^3_{a,\gamma} \quad (2r_T r_V N_v) \quad (7922)$$

$$\tau^2_{\gamma,\alpha,i} = \sum_{\beta \in B} W^1_{i,\beta} X_{\beta,\alpha} \tau^1_{\gamma,\beta} \quad (3r_T r_V^2 N_o) \quad (7923)$$

$$\tau^3_{\gamma,\alpha} = \sum_{i \in O} W^3_{i,\alpha} Y^4_{i,\gamma} \quad (2r_T r_V N_o) \quad (7924)$$

$$\tau^4_{\gamma,\alpha} = \sum_{a \in V} W^4_{a,\alpha} Y^3_{a,\gamma} \quad (2r_T r_V N_v) \quad (7925)$$

$$\tau^5_{\gamma,\delta,i} = \sum_{\alpha \in B} \tau^3_{\gamma,\alpha} \tau^4_{\delta,\alpha} \tau^2_{\gamma,\alpha,i} \quad (3r_T^2 r_V N_o) \quad (7926)$$

$$\tau^6_{\gamma,\delta,\epsilon} = \sum_{i \in O} Y^2_{i,\gamma} Z_{\gamma,\delta} \tau^5_{\epsilon,\delta,i} \quad (3r_T^3 N_o) \quad (7927)$$

$$\tau^7_{\gamma,\delta,i} = \sum_{\epsilon \in A} Y^4_{i,\epsilon} \tau^6_{\gamma,\epsilon,\delta} \quad (2r_T^3 N_o) \quad (7928)$$

$$\tau^8_{\gamma,\delta,w} = \sum_{\epsilon \in A} \sum_{i \in O} {}^2D^2_{i,w} Y^{2,*}_{i,\delta} \tau^0_{\epsilon,\delta,w} \tau^7_{\epsilon,\gamma,i} \quad (4r_D r_T^3 N_o) \quad (7929)$$

$$\tau^9_{\gamma,\delta,w} = \sum_{a \in V} {}^2D^3_{a,w} Y^1_{a,\gamma} Y^{3,*}_{a,\delta} \quad (3r_D r_T^2 N_v) \quad (7930)$$

$$\tau^{10}_{\gamma,\delta,w} = \sum_{i \in O} {}^2D^4_{i,w} Y^2_{i,\gamma} Y^{4,*}_{i,\delta} \quad (3r_D r_T^2 N_o) \quad (7931)$$

$$\tau^{11}_{\gamma,\delta,w} = \sum_{\epsilon \in A} Z_{\epsilon,\gamma} \tau^{10}_{\epsilon,\delta,w} \tau^9_{\epsilon,\delta,w} \quad (3r_D r_T^3) \quad (7932)$$

$${}^2R^z_{\gamma,\delta} \leftarrow \sum_{\epsilon \in A} \sum_{w \in D} \frac{1}{4} \tau^{11}_{\epsilon,\delta,w} \tau^8_{\epsilon,\gamma,w} \quad (2r_D r_T^3) \quad (7933)$$

Raw expression

$${}^2R^z_{\epsilon,\zeta} \leftarrow \sum_{i \in O} \sum_{j \in O} \sum_{k \in O} \sum_{l \in O} \sum_{a \in V} \sum_{b \in V} \sum_{c \in V} \sum_{d \in V} \frac{1}{4} Y^{1,*}_{a,\epsilon} Y^{2,*}_{i,\epsilon} Y^{3,*}_{b,\zeta} Y^{4,*}_{j,\zeta} {}^2D^{a,i,b,j} {}^2T_{a,k,d,i} {}^2T_{b,j,c,l} V_{k,c,l,d} \quad (7934)$$

Factorized expression

$$\tau^0_{\gamma,\delta,w} = \sum_{a \in V} {}^2D^3_{a,w} Y^3_{a,\gamma} Y^{3,*}_{a,\delta} \quad (3r_D r_T^2 N_v) \quad (7935)$$

$$\tau^1_{\gamma,\delta,w,i} = \sum_{\epsilon \in A} Z_{\gamma,\epsilon} Y^4_{i,\epsilon} \tau^0_{\epsilon,\delta,w} \quad (3r_D r_T^3 N_o) \quad (7936)$$

$$\tau^0_{\gamma,\delta,w} = \sum_{a \in V} {}^2D^1_{a,w} Y^1_{a,\gamma} Y^{1,*}_{a,\delta} \quad (3r_D r_T^2 N_v) \quad (7948)$$

$$\tau^2_{\gamma,\alpha} = \sum_{a \in V} W^2_{a,\alpha} Y^1_{a,\gamma} \quad (2r_T r_V N_v) \quad (7937)$$

$$\tau^1_{\gamma,\delta,w} = \sum_{a \in V} {}^2D^3_{a,w} Y^3_{a,\gamma} Y^{3,*}_{a,\delta} \quad (3r_D r_T^2 N_v) \quad (7949)$$

$$\tau^3_{\gamma,\alpha,i} = \sum_{\beta \in B} W^1_{i,\beta} X_{\beta,\alpha} \tau^2_{\gamma,\beta} \quad (3r_T r_V^2 N_o) \quad (7938)$$

$$\tau^2_{\gamma,\delta,w,i} = \sum_{\epsilon \in A} Z_{\gamma,\epsilon} Y^4_{i,\epsilon} \tau^1_{\epsilon,\delta,w} \quad (3r_D r_T^3 N_o) \quad (7950)$$

$$\tau^4_{\gamma,\alpha} = \sum_{a \in V} W^4_{a,\alpha} Y^3_{a,\gamma} \quad (2r_T r_V N_v) \quad (7939)$$

$$\tau^3_{\gamma,\delta,\alpha,w} = \sum_{i \in O} W^3_{i,\alpha} \tau^2_{\gamma,\delta,w,i} \quad (2r_D r_T^2 r_V N_o) \quad (7951)$$

$$\tau^5_{\gamma,\alpha,i} = \sum_{\delta \in A} Z_{\gamma,\delta} Y^4_{i,\delta} \tau^4_{\delta,\alpha} \quad (3r_T^2 r_V N_o) \quad (7940)$$

$$\tau^4_{\gamma,\alpha} = \sum_{a \in V} W^2_{a,\alpha} Y^1_{a,\gamma} \quad (2r_T r_V N_v) \quad (7952)$$

$$\tau^6_{\gamma,i,j,k} = \sum_{\alpha \in B} W^3_{j,\alpha} \tau^3_{\gamma,\alpha,i} \tau^5_{\gamma,\alpha,k} \quad (3r_T r_V N_o^3) \quad (7941)$$

$$\tau^5_{\gamma,\alpha,i} = \sum_{\beta \in B} W^1_{i,\beta} X_{\beta,\alpha} \tau^4_{\gamma,\beta} \quad (3r_T r_V^2 N_o) \quad (7953)$$

$$\tau^7_{i,j,k,l} = \sum_{\gamma \in A} Y^2_{k,\gamma} \tau^6_{\gamma,i,j,l} \quad (2r_T N_o^4) \quad (7942)$$

$$\tau^6_{\gamma,\delta,\alpha} = \sum_{i \in O} Y^2_{i,\delta} \tau^5_{\gamma,\alpha,i} \quad (2r_T^2 r_V N_o) \quad (7954)$$

$$\tau^8_{\gamma,i,j,k} = \sum_{l \in O} Y^2_{l,\gamma} \tau^7_{l,i,j,k} \quad (2r_T N_o^4) \quad (7943)$$

$$\tau^7_{\gamma,\alpha} = \sum_{a \in V} W^4_{a,\alpha} Y^3_{a,\gamma} \quad (2r_T r_V N_v) \quad (7955)$$

$$\tau^8_{\gamma,\alpha,i} = \sum_{\delta \in A} Z_{\gamma,\delta} Y^4_{i,\delta} \tau^7_{\delta,\alpha} \quad (3r_T^2 r_V N_o) \quad (7956)$$

$$\tau^9_{\gamma,\delta,w,i} = \sum_{j \in O} \sum_{k \in O} {}^2D^4_{j,w} Y^{4,*}_{j,\delta} \tau^1_{\gamma,\delta,w,k} \tau^8_{\gamma,k,i,j} \quad (4r_D r_T^2 N_o^3) \quad (7944)$$

$$\tau^9_{\gamma,\delta,\alpha,w} = \sum_{i \in O} {}^2D^4_{i,w} Y^{4,*}_{i,\delta} \tau^8_{\gamma,\alpha,i} \quad (3r_D r_T^2 r_V N_o) \quad (7957)$$

$$\tau^{10}_{\gamma,\delta,w} = \sum_{a \in V} {}^2D^1_{a,w} Y^1_{a,\gamma} Y^{1,*}_{a,\delta} \quad (3r_D r_T^2 N_v) \quad (7945)$$

$$\tau^{10}_{\gamma,\delta,\epsilon,w} = \sum_{\alpha \in B} \tau^6_{\gamma,\delta,\alpha} \tau^3_{\gamma,\epsilon,\alpha,w} \tau^9_{\delta,\epsilon,\alpha,w} \quad (3r_D r_T^3 r_V) \quad (7958)$$

$${}^2R^z_{\gamma,\delta} \leftarrow \sum_{\epsilon \in A} \sum_{w \in D} \sum_{i \in O} \frac{1}{4} {}^2D^2_{i,w} Y^{2,*}_{i,\gamma} \tau^{10}_{\epsilon,\gamma,w} \tau^9_{\epsilon,\delta,w,i} \quad (4r_D r_T^3 N_o) \quad (7946)$$

$$\tau^{11}_{\gamma,\delta,w,i} = \sum_{\epsilon \in A} {}^2D^2_{i,w} Y^2_{i,\epsilon} \tau^{10}_{\epsilon,\gamma,\delta,w} \quad (3r_D r_T^3 N_o) \quad (7959)$$

Raw expression

$${}^2R^z_{\epsilon,\zeta} \leftarrow \sum_{i \in O} \sum_{j \in O} \sum_{k \in O} \sum_{l \in O} \sum_{a \in V} \sum_{b \in V} \sum_{c \in V} \sum_{d \in V} \frac{1}{4} Y^{1,*}_{a,\epsilon} Y^{2,*}_{i,\epsilon} Y^{3,*}_{b,\zeta} Y^{4,*}_{j,\zeta} {}^2D^{a,i,b,j} {}^2T_{a,k,d,i} {}^2T_{c,j,b,l} V_{k,d,l,c} \quad (7947)$$

$$\tau^{12}_{\gamma,\delta,i} = \sum_{\epsilon \in A} \sum_{w \in D} \tau^0_{\epsilon,\gamma,w} \tau^{11}_{\epsilon,\delta,w,i} \quad (2r_D r_T^3 N_o) \quad (7960)$$

$${}^2R^z_{\gamma,\delta} \leftarrow \sum_{i \in O} \frac{1}{4} Y^{2,*}_{i,\gamma} \tau^{12}_{\gamma,\delta,i} \quad (2r_T^2 N_o) \quad (7961)$$

Factorized expression



Raw expression

$${}^2R^z_{\epsilon,\zeta} \leftarrow \sum_{i \in O} \sum_{j \in O} \sum_{k \in O} \sum_{l \in O} \sum_{a \in V} \sum_{b \in V} \sum_{c \in V} \sum_{d \in V} \frac{1}{4} Y^{1,*}_{a,\epsilon} Y^{2,*}_{i,\epsilon} Y^{3,*}_{b,\zeta} Y^{4,*}_{j,\zeta} {}^2D^{a,i,b,j} {}^2T_{a,k,d,j} {}^2T_{b,l,c,i} V_{k,c,l,d} \quad (7962)$$

Factorized expression

$$\tau^0_{\gamma,\delta,w} = \sum_{i \in O} {}^2D^2_{i,w} Y^2_{i,\gamma} Y^{2,*}_{i,\delta} \quad (3r_D r_T^2 N_o) \quad (7963)$$

$$\tau^1_{\gamma,\alpha} = \sum_{a \in V} W^2_{a,\alpha} Y^3_{a,\gamma} \quad (2r_T r_V N_v) \quad (7964)$$

$$\tau^2_{\gamma,\alpha,i} = \sum_{\beta \in B} W^1_{i,\beta} X_{\beta,\alpha} \tau^1_{\gamma,\beta} \quad (3r_T r_V^2 N_o) \quad (7965)$$

$$\tau^3_{\gamma,\alpha} = \sum_{i \in O} W^3_{i,\alpha} Y^4_{i,\gamma} \quad (2r_T r_V N_o) \quad (7966)$$

$$\tau^4_{\gamma,\alpha} = \sum_{\delta \in A} \sum_{i \in O} Y^2_{i,\gamma} Z_{\gamma,\delta} \tau^3_{\delta,\alpha} \tau^2_{\delta,\alpha,i} \quad (4r_T^2 r_V N_o) \quad (7967)$$

$$\tau^5_{\gamma,a} = \sum_{\alpha \in B} W^4_{a,\alpha} \tau^4_{\gamma,\alpha} \quad (2r_T r_V N_v) \quad (7968)$$

$$\tau^6_{\gamma,\delta} = \sum_{a \in V} Y^1_{a,\gamma} \tau^5_{\delta,a} \quad (2r_T^2 N_v) \quad (7969)$$

$$\tau^7_{\gamma,a} = \sum_{\delta \in A} Y^1_{a,\delta} \tau^6_{\gamma,\delta} \quad (2r_T^2 N_v) \quad (7970)$$

$$\tau^8_{\gamma,\delta,w} = \sum_{a \in V} {}^2D^1_{a,w} Y^{1,*}_{a,\delta} \tau^7_{\gamma,a} \quad (3r_D r_T^2 N_v) \quad (7971)$$

$$\tau^9_{\gamma,\delta,w} = \sum_{\epsilon \in A} Z_{\epsilon,\gamma} \tau^0_{\epsilon,\delta,w} \tau^8_{\epsilon,\delta,w} \quad (3r_D r_T^3) \quad (7972)$$

$$\tau^{10}_{\gamma,\delta,w} = \sum_{a \in V} {}^2D^3_{a,w} Y^3_{a,\gamma} Y^{3,*}_{a,\delta} \quad (3r_D r_T^2 N_v) \quad (7973)$$

$$\tau^{11}_{\gamma,\delta,w} = \sum_{i \in O} {}^2D^4_{i,w} Y^4_{i,\gamma} Y^{4,*}_{i,\delta} \quad (3r_D r_T^2 N_o) \quad (7974)$$

$${}^2R^z_{\gamma,\delta} \leftarrow \sum_{\epsilon \in A} \sum_{w \in D} \frac{1}{4} \tau^{10}_{\epsilon,\delta,w} \tau^{11}_{\epsilon,\delta,w} \tau^9_{\epsilon,\gamma,w} \quad (3r_D r_T^3) \quad (7975)$$

Raw expression

$${}^2R^z_{\epsilon,\zeta} \leftarrow \sum_{i \in O} \sum_{j \in O} \sum_{k \in O} \sum_{l \in O} \sum_{a \in V} \sum_{b \in V} \sum_{c \in V} \sum_{d \in V} \frac{1}{4} Y^{1,*}_{a,\epsilon} Y^{2,*}_{i,\epsilon} Y^{3,*}_{b,\zeta} Y^{4,*}_{j,\zeta} {}^2D^{a,i,b,j} {}^2T_{a,k,d,j} {}^2T_{c,i,b,l} V_{k,c,l,d} \quad (7976)$$

Factorized expression

$$\tau^0_{\gamma,\alpha} = \sum_{a \in V} W^2_{a,\alpha} Y^3_{a,\gamma} \quad (2r_T r_V N_v) \quad (7977)$$

$$\tau^1_{\gamma,\alpha,i} = \sum_{\beta \in B} W^1_{i,\beta} X_{\beta,\alpha} \tau^0_{\gamma,\beta} \quad (3r_T r_V^2 N_o) \quad (7978)$$

$$\tau^2_{\gamma,\alpha} = \sum_{i \in O} W^3_{i,\alpha} Y^4_{i,\gamma} \quad (2r_T r_V N_o) \quad (7979)$$

$$\tau^3_{\gamma,\alpha} = \sum_{a \in V} W^4_{a,\alpha} Y^1_{a,\gamma} \quad (2r_T r_V N_v) \quad (7980)$$

$$\tau^4_{\gamma,\delta,i} = \sum_{\alpha \in B} \tau^2_{\delta,\alpha} \tau^3_{\gamma,\alpha} \tau^1_{\delta,\alpha,i} \quad (3r_T^2 r_V N_o) \quad (7981)$$

$$\tau^5_{\gamma,i} = \sum_{\delta \in A} Z_{\gamma,\delta} \tau^4_{\gamma,\delta,i} \quad (2r_T^2 N_o) \quad (7982)$$

$$\tau^6_{i,j} = \sum_{\gamma \in A} Y^2_{j,\gamma} \tau^5_{\gamma,i} \quad (2r_T N_o^2) \quad (7983)$$

$$\tau^7_{\gamma,i} = \sum_{j \in O} Y^2_{j,\gamma} \tau^6_{j,i} \quad (2r_T N_o^2) \quad (7984)$$

$$\tau^8_{\gamma,\delta,w} = \sum_{i \in O} {}^2D^2_{i,w} Y^{2,*}_{i,\delta} \tau^7_{\gamma,i} \quad (3r_D r_T^2 N_o) \quad (7985)$$

$$\tau^9_{\gamma,\delta,w} = \sum_{a \in V} {}^2D^1_{a,w} Y^1_{a,\gamma} Y^{1,*}_{a,\delta} \quad (3r_D r_T^2 N_v) \quad (7986)$$

$$\tau^{10}_{\gamma,\delta,w} = \sum_{a \in V} {}^2D^3_{a,w} Y^3_{a,\gamma} Y^{3,*}_{a,\delta} \quad (3r_D r_T^2 N_v) \quad (7987)$$

$$\tau^{11}_{\gamma,\delta,w} = \sum_{i \in O} {}^2D^4_{i,w} Y^4_{i,\gamma} Y^{4,*}_{i,\delta} \quad (3r_D r_T^2 N_o) \quad (7988)$$

$$\tau^9_{\gamma,i,j,k} = \sum_{l \in O} Y^2_{l,\gamma} \tau^8_{l,i,j,k} \quad (2r_T N_o^4) \quad (8001)$$

$$\tau^{12}_{\gamma,\delta,w} = \sum_{\epsilon \in A} Z_{\gamma,\epsilon} \tau^{10}_{\epsilon,\delta,w} \tau^{11}_{\epsilon,\delta,w} \quad (3r_D r_T^3) \quad (7989)$$

$$\tau^{10}_{\gamma,\delta,w,i} = \sum_{j \in O} \sum_{k \in O} {}^2D^4_{j,w} Y^{4,*}_{j,\delta} \tau^2_{\gamma,\delta,w,k} \tau^9_{\gamma,k,j,i} \quad (4r_D r_T^2 N_o^3) \quad (8002)$$

$${}^2R^z_{\gamma,\delta} \leftarrow \sum_{\epsilon \in A} \sum_{w \in D} \frac{1}{4} \tau^{12}_{\epsilon,\delta,w} \tau^8_{\epsilon,\gamma,w} \tau^9_{\epsilon,\gamma,w} \quad (3r_D r_T^3) \quad (7990)$$

$${}^2R^z_{\gamma,\delta} \leftarrow \sum_{\epsilon \in A} \sum_{w \in D} \sum_{i \in O} \frac{1}{4} {}^2D^2_{i,w} Y^{2,*}_{i,\gamma} \tau^0_{\epsilon,\gamma,w} \tau^{10}_{\epsilon,\delta,w,i} \quad (4r_D r_T^3 N_o) \quad (8003)$$

Raw expression

$${}^2R^z_{\epsilon,\zeta} \leftarrow \sum_{i \in O} \sum_{j \in O} \sum_{k \in O} \sum_{l \in O} \sum_{a \in V} \sum_{b \in V} \sum_{c \in V} \sum_{d \in V} \frac{1}{4} Y^{1,*}_{a,\epsilon} Y^{2,*}_{i,\epsilon} Y^{3,*}_{b,\zeta} Y^{4,*}_{j,\zeta} {}^2D^{a,i,b,j} {}^2T_{a,k,d,l} {}^2T_{b,j,c,i} V_{k,d,l,c} \quad (7991)$$

Raw expression

$${}^2R^z_{\epsilon,\zeta} \leftarrow \sum_{i \in O} \sum_{j \in O} \sum_{k \in O} \sum_{l \in O} \sum_{a \in V} \sum_{b \in V} \sum_{c \in V} \sum_{d \in V} \frac{1}{4} Y^{1,*}_{a,\epsilon} Y^{2,*}_{i,\epsilon} Y^{3,*}_{b,\zeta} Y^{4,*}_{j,\zeta} {}^2D^{a,i,b,j} {}^2T_{a,k,d,l} {}^2T_{c,i,b,j} V_{k,d,l,c} \quad (8004)$$

Factorized expression

$$\tau^0_{\gamma,\delta,w} = \sum_{a \in V} {}^2D^1_{a,w} Y^1_{a,\gamma} Y^{1,*}_{a,\delta} \quad (3r_D r_T^2 N_v) \quad (7992)$$

$$\tau^0_{\gamma,\delta,w} = \sum_{a \in V} {}^2D^1_{a,w} Y^1_{a,\gamma} Y^{1,*}_{a,\delta} \quad (3r_D r_T^2 N_v) \quad (8005)$$

$$\tau^1_{\gamma,\delta,w} = \sum_{a \in V} {}^2D^3_{a,w} Y^3_{a,\gamma} Y^{3,*}_{a,\delta} \quad (3r_D r_T^2 N_v) \quad (7993)$$

$$\tau^1_{\gamma,\alpha} = \sum_{i \in O} W^1_{i,\alpha} Y^2_{i,\gamma} \quad (2r_T r_V N_o) \quad (8006)$$

$$\tau^2_{\gamma,\delta,w,i} = \sum_{\epsilon \in A} Z_{\gamma,\epsilon} Y^4_{i,\epsilon} \tau^1_{\epsilon,\delta,w} \quad (3r_D r_T^3 N_o) \quad (7994)$$

$$\tau^2_{\gamma,\alpha} = \sum_{a \in V} W^2_{a,\alpha} Y^3_{a,\gamma} \quad (2r_T r_V N_v) \quad (8007)$$

$$\tau^3_{\gamma,\alpha} = \sum_{a \in V} W^4_{a,\alpha} Y^1_{a,\gamma} \quad (2r_T r_V N_v) \quad (7995)$$

$$\tau^3_{\gamma,\alpha,i} = \sum_{\delta \in A} Z_{\gamma,\delta} Y^4_{i,\delta} \tau^2_{\delta,\alpha} \quad (3r_T^2 r_V N_o) \quad (8008)$$

$$\tau^4_{\gamma,\alpha,i} = \sum_{\beta \in B} X_{\alpha,\beta} W^3_{i,\beta} \tau^3_{\gamma,\beta} \quad (3r_T r_V^2 N_o) \quad (7996)$$

$$\tau^4_{\gamma,\alpha,w} = \sum_{\delta \in A} \sum_{i \in O} {}^2D^2_{i,w} Y^{2,*}_{i,\gamma} \tau^1_{\delta,\alpha} \tau^0_{\delta,\gamma,w} \tau^3_{\delta,\alpha,i} \quad (5r_D r_T^2 r_V N_o) \quad (8009)$$

$$\tau^5_{\gamma,\alpha} = \sum_{a \in V} W^2_{a,\alpha} Y^3_{a,\gamma} \quad (2r_T r_V N_v) \quad (7997)$$

$$\tau^5_{\gamma,\alpha,w} = \sum_{\beta \in B} X_{\beta,\alpha} \tau^4_{\gamma,\beta,w} \quad (2r_D r_T r_V^2) \quad (8010)$$

$$\tau^6_{\gamma,\alpha,i} = \sum_{\delta \in A} Z_{\gamma,\delta} Y^4_{i,\delta} \tau^5_{\delta,\alpha} \quad (3r_T^2 r_V N_o) \quad (7998)$$

$$\tau^6_{\gamma,\delta,w} = \sum_{a \in V} {}^2D^3_{a,w} Y^3_{a,\gamma} Y^{3,*}_{a,\delta} \quad (3r_D r_T^2 N_v) \quad (8011)$$

$$\tau^7_{\gamma,i,j,k} = \sum_{\alpha \in B} W^1_{i,\alpha} \tau^4_{\gamma,\alpha,j} \tau^6_{\gamma,\alpha,k} \quad (3r_T r_V N_o^3) \quad (7999)$$

$$\tau^7_{\gamma,\alpha} = \sum_{a \in V} W^4_{a,\alpha} Y^1_{a,\gamma} \quad (2r_T r_V N_v) \quad (8012)$$

$$\tau^8_{i,j,k,l} = \sum_{\gamma \in A} Y^2_{k,\gamma} \tau^7_{\gamma,i,j,l} \quad (2r_T N_o^4) \quad (8000)$$

$$\tau^8_{\gamma,\alpha,i} = \sum_{\delta \in A} Y^2_{i,\delta} Z_{\delta,\gamma} \tau^7_{\delta,\alpha} \quad (3r_T^2 r_V N_o) \quad (8013)$$

$$\tau^9_{\gamma,\alpha} = \sum_{i \in O} W^3_{i,\alpha} Y^4_{i,\gamma} \quad (2r_T r_V N_o) \quad (8014)$$

$$\tau^9_{\gamma,\delta,w} = \sum_{i \in O} {}^2D^2_{i,w} Y^{2,*}_{i,\delta} \tau^8_{\gamma,i} \quad (3r_D r_T^2 N_o) \quad (8027)$$

$$\tau^{10}_{\gamma,\alpha,w} = \sum_{\delta \in A} \sum_{i \in O} {}^2D^4_{i,w} Y^{4,*}_{i,\gamma} \tau^9_{\delta,\alpha} \tau^6_{\delta,\gamma,w} \tau^8_{\delta,\alpha,i} \quad (5r_D r_T^2 r_V N_o^{10}) \quad (8015)$$

$$\tau^{10}_{\gamma,\delta,w} = \sum_{\epsilon \in A} Z_{\gamma,\epsilon} \tau^0_{\epsilon,\delta,w} \tau^9_{\epsilon,\delta,w} \quad (3r_D r_T^3) \quad (8028)$$

$${}^2R^z_{\gamma,\delta} \leftarrow \sum_{\alpha \in B} \sum_{w \in D} \frac{1}{4} \tau^{10}_{\delta,\alpha,w} \tau^5_{\gamma,\alpha,w} \quad (2r_D r_T^2 r_V) \quad (8016)$$

$$\tau^{11}_{\gamma,\delta,w} = \sum_{a \in V} {}^2D^3_{a,w} Y^1_{a,\gamma} Y^{3,*}_{a,\delta} \quad (3r_D r_T^2 N_v) \quad (8029)$$

Raw expression

$${}^2R^z_{\epsilon,\zeta} \leftarrow \sum_{i \in O} \sum_{j \in O} \sum_{k \in O} \sum_{l \in O} \sum_{a \in V} \sum_{b \in V} \sum_{c \in V} \sum_{d \in V} \frac{1}{4} Y^{1,*}_{a,\epsilon} Y^{2,*}_{i,\epsilon} Y^{3,*}_{b,\zeta} Y^{4,*}_{j,\zeta} {}^2D^{a,i,b,j} {}^2T_{b,j,a,k} {}^2T_{c,i,d,l} V_{k,d,l,c} \quad (8017)$$

$$\tau^{12}_{\gamma,\delta,w} = \sum_{i \in O} {}^2D^4_{i,w} Y^2_{i,\gamma} Y^{4,*}_{i,\delta} \quad (3r_D r_T^2 N_o) \quad (8030)$$

$${}^2R^z_{\gamma,\delta} \leftarrow \sum_{\epsilon \in A} \sum_{w \in D} \frac{1}{4} \tau^{10}_{\epsilon,\gamma,w} \tau^{11}_{\epsilon,\delta,w} \tau^{12}_{\epsilon,\delta,w} \quad (3r_D r_T^3) \quad (8031)$$

Factorized expression

$$\tau^0_{\gamma,\delta,w} = \sum_{a \in V} {}^2D^1_{a,w} Y^3_{a,\gamma} Y^{1,*}_{a,\delta} \quad (3r_D r_T^2 N_v) \quad (8018)$$

Raw expression

$${}^2R^z_{\epsilon,\zeta} \leftarrow \sum_{i \in O} \sum_{j \in O} \sum_{k \in O} \sum_{l \in O} \sum_{a \in V} \sum_{b \in V} \sum_{c \in V} \sum_{d \in V} \frac{1}{4} Y^{1,*}_{a,\epsilon} Y^{2,*}_{i,\epsilon} Y^{3,*}_{b,\zeta} Y^{4,*}_{j,\zeta} {}^2D^{a,i,b,j} {}^2T_{b,j,a,l} {}^2T_{c,k,d,i} V_{l,c,k,d} \quad (8032)$$

$$\tau^1_{\gamma,\alpha} = \sum_{a \in V} W^2_{a,\alpha} Y^1_{a,\gamma} \quad (2r_T r_V N_v) \quad (8019)$$

Factorized expression

$$\tau^2_{\gamma,\alpha,i} = \sum_{\beta \in B} W^1_{i,\beta} X_{\beta,\alpha} \tau^1_{\gamma,\beta} \quad (3r_T r_V^2 N_o) \quad (8020)$$

$$\tau^0_{\gamma,\delta,w} = \sum_{a \in V} {}^2D^1_{a,w} Y^3_{a,\gamma} Y^{1,*}_{a,\delta} \quad (3r_D r_T^2 N_v) \quad (8033)$$

$$\tau^3_{\gamma,\alpha} = \sum_{i \in O} W^3_{i,\alpha} Y^2_{i,\gamma} \quad (2r_T r_V N_o) \quad (8021)$$

$$\tau^1_{\gamma,\delta,w} = \sum_{i \in O} {}^2D^2_{i,w} Y^4_{i,\gamma} Y^{2,*}_{i,\delta} \quad (3r_D r_T^2 N_o) \quad (8034)$$

$$\tau^4_{\gamma,\alpha} = \sum_{a \in V} W^4_{a,\alpha} Y^3_{a,\gamma} \quad (2r_T r_V N_v) \quad (8022)$$

$$\tau^2_{\gamma,\delta,w} = \sum_{\epsilon \in A} Z_{\gamma,\epsilon} \tau^0_{\epsilon,\delta,w} \tau^1_{\epsilon,\delta,w} \quad (3r_D r_T^3) \quad (8035)$$

$$\tau^5_{\gamma,\delta,i} = \sum_{\alpha \in B} \tau^3_{\gamma,\alpha} \tau^4_{\delta,\alpha} \tau^2_{\gamma,\alpha,i} \quad (3r_T^2 r_V N_o) \quad (8023)$$

$$\tau^3_{\gamma,\alpha} = \sum_{a \in V} W^2_{a,\alpha} Y^1_{a,\gamma} \quad (2r_T r_V N_v) \quad (8036)$$

$$\tau^6_{\gamma,i} = \sum_{\delta \in A} Z_{\delta,\gamma} \tau^5_{\delta,\gamma,i} \quad (2r_T^2 N_o) \quad (8024)$$

$$\tau^4_{\gamma,\alpha,i} = \sum_{\beta \in B} W^1_{i,\beta} X_{\beta,\alpha} \tau^3_{\gamma,\beta} \quad (3r_T r_V^2 N_o) \quad (8037)$$

$$\tau^7_{i,j} = \sum_{\gamma \in A} Y^4_{j,\gamma} \tau^6_{\gamma,i} \quad (2r_T N_o^2) \quad (8025)$$

$$\tau^5_{\gamma,\alpha} = \sum_{i \in O} W^3_{i,\alpha} Y^2_{i,\gamma} \quad (2r_T r_V N_o) \quad (8038)$$

$$\tau^8_{\gamma,i} = \sum_{j \in O} Y^4_{j,\gamma} \tau^7_{j,i} \quad (2r_T N_o^2) \quad (8026)$$

$$\tau^6_{\gamma,\alpha} = \sum_{a \in V} W^4_{a,\alpha} Y^3_{a,\gamma} \quad (2r_T r_V N_v) \quad (8039)$$

$$\tau_{\gamma,\delta,i}^7 = \sum_{\alpha \in B} \tau_{\gamma,\alpha}^5 \tau_{\delta,\alpha}^6 \tau_{\gamma,\alpha,i}^4 \quad (3r_T^2 r_V N_o) \quad (8040)$$

$$\tau_{\gamma,i}^8 = \sum_{\delta \in A} Z_{\delta,\gamma} \tau_{\delta,\gamma,i}^7 \quad (2r_T^2 N_o) \quad (8041)$$

$$\tau_{i,j}^9 = \sum_{\gamma \in A} Y_{j,\gamma}^4 \tau_{\gamma,i}^8 \quad (2r_T N_o^2) \quad (8042)$$

$$\tau_{\gamma,i}^{10} = \sum_{j \in O} Y_{j,\gamma}^2 \tau_{j,i}^9 \quad (2r_T N_o^2) \quad (8043)$$

$$\tau_{\gamma,\delta,w}^{11} = \sum_{i \in O} {}^2D_{i,w}^4 Y_{i,\delta}^{4,*} \tau_{\gamma,i}^{10} \quad (3r_D r_T^2 N_o) \quad (8044)$$

$$\tau_{\gamma,\delta,w}^{12} = \sum_{a \in V} {}^2D_{a,w}^3 Y_{a,\gamma}^1 Y_{a,\delta}^{3,*} \quad (3r_D r_T^2 N_v) \quad (8045)$$

$${}^2R_{\gamma,\delta}^z \leftarrow \sum_{\epsilon \in A} \sum_{w \in D} \frac{1}{4} \tau_{\epsilon,\delta,w}^{11} \tau_{\epsilon,\delta,w}^{12} \tau_{\epsilon,\gamma,w}^2 \quad (3r_D r_T^3) \quad (8046)$$

Raw expression

$${}^2R_{\epsilon,\zeta}^z \leftarrow \sum_{i \in O} \sum_{j \in O} \sum_{k \in O} \sum_{l \in O} \sum_{a \in V} \sum_{b \in V} \sum_{c \in V} \sum_{d \in V} \frac{1}{4} Y_{a,\epsilon}^{1,*} Y_{i,\epsilon}^{2,*} Y_{b,\zeta}^{3,*} Y_{j,\zeta}^{4,*} {}^2D_{a,i,b,j} {}^2T_{b,j,c,i} {}^2T_{d,k,a,l} V_{k,c,l,d} \quad (8047)$$

Factorized expression

$$\tau_{\gamma,\delta,w}^0 = \sum_{a \in V} {}^2D_{a,w}^1 Y_{a,\gamma}^3 Y_{a,\delta}^{1,*} \quad (3r_D r_T^2 N_v) \quad (8048)$$

$$\tau_{\gamma,\alpha}^1 = \sum_{a \in V} W_{a,\alpha}^2 Y_{a,\gamma}^3 \quad (2r_T r_V N_v) \quad (8049)$$

$$\tau_{\gamma,\alpha,i}^2 = \sum_{\beta \in B} W_{i,\beta}^1 X_{\beta,\alpha} \tau_{\gamma,\beta}^1 \quad (3r_T r_V^2 N_o) \quad (8050)$$

$$\tau_{\gamma,\alpha}^3 = \sum_{i \in O} W_{i,\alpha}^3 Y_{i,\gamma}^4 \quad (2r_T r_V N_o) \quad (8051)$$

$$\tau_{\gamma,\alpha}^4 = \sum_{a \in V} W_{a,\alpha}^4 Y_{a,\gamma}^1 \quad (2r_T r_V N_v) \quad (8052)$$

$$\tau_{\gamma,\delta,i}^5 = \sum_{\alpha \in B} \tau_{\delta,\alpha}^3 \tau_{\gamma,\alpha}^4 \tau_{\delta,\alpha,i}^2 \quad (3r_T^2 r_V N_o) \quad (8053)$$

$$\tau_{\gamma,i}^6 = \sum_{\delta \in A} Z_{\gamma,\delta} \tau_{\gamma,\delta,i}^5 \quad (2r_T^2 N_o) \quad (8054)$$

$$\tau_{i,j}^7 = \sum_{\gamma \in A} Y_{j,\gamma}^2 \tau_{\gamma,i}^6 \quad (2r_T N_o^2) \quad (8055)$$

$$\tau_{\gamma,i}^8 = \sum_{j \in O} Y_{j,\gamma}^4 \tau_{j,i}^7 \quad (2r_T N_o^2) \quad (8056)$$

$$\tau_{\gamma,\delta,w}^9 = \sum_{i \in O} {}^2D_{i,w}^2 Y_{i,\delta}^{2,*} \tau_{\gamma,i}^8 \quad (3r_D r_T^2 N_o) \quad (8057)$$

$$\tau_{\gamma,\delta,w}^{10} = \sum_{\epsilon \in A} Z_{\gamma,\epsilon} \tau_{\epsilon,\delta,w}^0 \tau_{\epsilon,\delta,w}^9 \quad (3r_D r_T^3) \quad (8058)$$

$$\tau_{\gamma,\delta,w}^{11} = \sum_{a \in V} {}^2D_{a,w}^3 Y_{a,\gamma}^1 Y_{a,\delta}^{3,*} \quad (3r_D r_T^2 N_v) \quad (8059)$$

$$\tau_{\gamma,\delta,w}^{12} = \sum_{i \in O} {}^2D_{i,w}^4 Y_{i,\gamma}^2 Y_{i,\delta}^{4,*} \quad (3r_D r_T^2 N_o) \quad (8060)$$

$${}^2R_{\gamma,\delta}^z \leftarrow \sum_{\epsilon \in A} \sum_{w \in D} \frac{1}{4} \tau_{\epsilon,\gamma,w}^{10} \tau_{\epsilon,\delta,w}^{11} \tau_{\epsilon,\delta,w}^{12} \quad (3r_D r_T^3) \quad (8061)$$

Raw expression

$${}^2R_{\epsilon,\zeta}^z \leftarrow \sum_{i \in O} \sum_{j \in O} \sum_{k \in O} \sum_{l \in O} \sum_{a \in V} \sum_{b \in V} \sum_{c \in V} \sum_{d \in V} \frac{1}{4} Y_{a,\epsilon}^{1,*} Y_{i,\epsilon}^{2,*} Y_{b,\zeta}^{3,*} Y_{j,\zeta}^{4,*} {}^2D_{a,i,b,j} {}^2T_{b,j,d,l} {}^2T_{c,i,a,k} V_{k,d,l,c} \quad (8062)$$

Factorized expression

$$\tau_{\gamma,\delta,w}^0 = \sum_{a \in V} {}^2D_{a,w}^1 Y_{a,\gamma}^3 Y_{a,\delta}^{1,*} \quad (3r_D r_T^2 N_v) \quad (8063)$$

$$\tau_{\gamma,\alpha}^1 = \sum_{a \in V} W_{a,\alpha}^2 Y_{a,\gamma}^3 \quad (2r_T r_V N_v) \quad (8064)$$

$$\tau_{\gamma,\alpha,i}^2 = \sum_{\beta \in B} W_{i,\beta}^1 X_{\beta,\alpha} \tau_{\gamma,\beta}^1 \quad (3r_T r_V^2 N_o) \quad (8065)$$

$$\tau^3_{\gamma,\alpha} = \sum_{i \in O} W^3_{i,\alpha} Y^4_{i,\gamma} \quad (2r_T r_V N_o) \quad (8066)$$

$$\tau^4_{\gamma,\alpha} = \sum_{a \in V} W^4_{a,\alpha} Y^1_{a,\gamma} \quad (2r_T r_V N_v) \quad (8067)$$

$$\tau^5_{\gamma,\delta,i} = \sum_{\alpha \in B} \tau^3_{\delta,\alpha} \tau^4_{\gamma,\alpha} \tau^2_{\delta,\alpha,i} \quad (3r_T^2 r_V N_o) \quad (8068)$$

$$\tau^6_{\gamma,\delta,\epsilon} = \sum_{i \in O} Z_{\gamma,\delta} Y^4_{i,\delta} \tau^5_{\gamma,\epsilon,i} \quad (3r_T^3 N_o) \quad (8069)$$

$$\tau^7_{\gamma,\delta,i} = \sum_{\epsilon \in A} Y^2_{i,\epsilon} \tau^6_{\epsilon,\gamma,\delta} \quad (2r_T^3 N_o) \quad (8070)$$

$$\tau^8_{\gamma,\delta,w} = \sum_{\epsilon \in A} \sum_{i \in O} {}^2D^2_{i,w} Y^{2,*}_{i,\delta} \tau^0_{\epsilon,\delta,w} \tau^7_{\epsilon,\gamma,i} \quad (4r_D r_T^3 N_o) \quad (8071)$$

$$\tau^9_{\gamma,\delta,w} = \sum_{\epsilon \in A} Z_{\gamma,\epsilon} \tau^8_{\epsilon,\delta,w} \quad (2r_D r_T^3) \quad (8072)$$

$$\tau^{10}_{\gamma,\delta,w} = \sum_{a \in V} {}^2D^3_{a,w} Y^1_{a,\gamma} Y^{3,*}_{a,\delta} \quad (3r_D r_T^2 N_v) \quad (8073)$$

$$\tau^{11}_{\gamma,\delta,w} = \sum_{i \in O} {}^2D^4_{i,w} Y^2_{i,\gamma} Y^{4,*}_{i,\delta} \quad (3r_D r_T^2 N_o) \quad (8074)$$

$${}^2R^z_{\gamma,\delta} \leftarrow \sum_{\epsilon \in A} \sum_{w \in D} \frac{1}{4} \tau^{10}_{\epsilon,\delta,w} \tau^{11}_{\epsilon,\delta,w} \tau^9_{\epsilon,\gamma,w} \quad (3r_D r_T^3) \quad (8075)$$

Raw expression

$${}^2R^z_{\epsilon,\zeta} \leftarrow \sum_{i \in O} \sum_{j \in O} \sum_{k \in O} \sum_{l \in O} \sum_{a \in V} \sum_{b \in V} \sum_{c \in V} \sum_{d \in V} \frac{1}{4} Y^{1,*}_{a,\epsilon} Y^{2,*}_{i,\epsilon} Y^{3,*}_{b,\zeta} Y^{4,*}_{j,\zeta} {}^2D^{a,i,b,j} {}^2T_{b,k,a,i} {}^2T_{c,j,d,l} V_{k,d,l,c} \quad (8076)$$

Factorized expression

$$\tau^0_{\gamma,\alpha} = \sum_{a \in V} W^4_{a,\alpha} Y^1_{a,\gamma} \quad (2r_T r_V N_v) \quad (8077)$$

$$\tau^1_{\gamma,\alpha,i} = \sum_{\beta \in B} X_{\alpha,\beta} W^3_{i,\beta} \tau^0_{\gamma,\beta} \quad (3r_T r_V^2 N_o) \quad (8078)$$

$$\tau^2_{\gamma,\alpha} = \sum_{i \in O} W^1_{i,\alpha} Y^2_{i,\gamma} \quad (2r_T r_V N_o) \quad (8079)$$

$$\tau^3_{\gamma,\alpha} = \sum_{\delta \in A} \sum_{i \in O} Z_{\delta,\gamma} Y^4_{i,\gamma} \tau^2_{\delta,\alpha} \tau^1_{\delta,\alpha,i} \quad (4r_T^2 r_V N_o) \quad (8080)$$

$$\tau^4_{\gamma,a} = \sum_{\alpha \in B} W^2_{a,\alpha} \tau^3_{\gamma,\alpha} \quad (2r_T r_V N_v) \quad (8081)$$

$$\tau^5_{a,b} = \sum_{\gamma \in A} Y^3_{b,\gamma} \tau^4_{\gamma,a} \quad (2r_T N_v^2) \quad (8082)$$

$$\tau^6_{\gamma,a} = \sum_{b \in V} Y^3_{b,\gamma} \tau^5_{b,a} \quad (2r_T N_v^2) \quad (8083)$$

$$\tau^7_{\gamma,\delta,w} = \sum_{a \in V} {}^2D^1_{a,w} Y^{1,*}_{a,\delta} \tau^6_{\gamma,a} \quad (3r_D r_T^2 N_v) \quad (8084)$$

$$\tau^8_{\gamma,\delta,w} = \sum_{i \in O} {}^2D^2_{i,w} Y^4_{i,\gamma} Y^{2,*}_{i,\delta} \quad (3r_D r_T^2 N_o) \quad (8085)$$

$$\tau^9_{\gamma,\delta,w} = \sum_{\epsilon \in A} Z_{\gamma,\epsilon} \tau^7_{\epsilon,\delta,w} \tau^8_{\epsilon,\delta,w} \quad (3r_D r_T^3) \quad (8086)$$

$$\tau^{10}_{\gamma,\delta,w} = \sum_{a \in V} {}^2D^3_{a,w} Y^1_{a,\gamma} Y^{3,*}_{a,\delta} \quad (3r_D r_T^2 N_v) \quad (8087)$$

$$\tau^{11}_{\gamma,\delta,w} = \sum_{i \in O} {}^2D^4_{i,w} Y^2_{i,\gamma} Y^{4,*}_{i,\delta} \quad (3r_D r_T^2 N_o) \quad (8088)$$

$${}^2R^z_{\gamma,\delta} \leftarrow \sum_{\epsilon \in A} \sum_{w \in D} \frac{1}{4} \tau^{10}_{\epsilon,\delta,w} \tau^{11}_{\epsilon,\delta,w} \tau^9_{\epsilon,\gamma,w} \quad (3r_D r_T^3) \quad (8089)$$

Raw expression

$${}^2R^z_{\epsilon,\zeta} \leftarrow \sum_{i \in O} \sum_{j \in O} \sum_{k \in O} \sum_{l \in O} \sum_{a \in V} \sum_{b \in V} \sum_{c \in V} \sum_{d \in V} \frac{1}{4} Y^{1,*}_{a,\epsilon} Y^{2,*}_{i,\epsilon} Y^{3,*}_{b,\zeta} Y^{4,*}_{j,\zeta} {}^2D^{a,i,b,j} {}^2T_{b,k,a,i} {}^2T_{c,l,d,j} V_{k,c,l,d} \quad (8090)$$

Factorized expression

$$\tau^0_{\gamma,\delta,w} = \sum_{a \in V} {}^2D^1_{a,w} Y^3_{a,\gamma} Y^{1,*}_{a,\delta} \quad (3r_D r_T^2 N_v) \quad (8091)$$

$$\tau^1_{\gamma,\delta,w} = \sum_{i \in O} {}^2D^2_{i,w} Y^4_{i,\gamma} Y^{2,*}_{i,\delta} \quad (3r_D r_T^2 N_o) \quad (8092)$$

$$\tau^0_{\gamma,\delta,w} = \sum_{a \in V} {}^2D^1_{a,w} Y^3_{a,\gamma} Y^{1,*}_{a,\delta} \quad (3r_D r_T^2 N_v) \quad (8105)$$

$$\tau^2_{\gamma,\delta,w} = \sum_{a \in V} {}^2D^3_{a,w} Y^1_{a,\gamma} Y^{3,*}_{a,\delta} \quad (3r_D r_T^2 N_v) \quad (8093)$$

$$\tau^1_{\gamma,\alpha} = \sum_{a \in V} W^2_{a,\alpha} Y^1_{a,\gamma} \quad (2r_T r_V N_v) \quad (8106)$$

$$\tau^3_{\gamma,\alpha} = \sum_{a \in V} W^4_{a,\alpha} Y^1_{a,\gamma} \quad (2r_T r_V N_v) \quad (8094)$$

$$\tau^2_{\gamma,\alpha,i} = \sum_{\delta \in A} Y^2_{i,\delta} Z_{\delta,\gamma} \tau^1_{\delta,\alpha} \quad (3r_T^2 r_V N_o) \quad (8107)$$

$$\tau^4_{\gamma,\alpha,i} = \sum_{\beta \in B} X_{\alpha,\beta} W^3_{i,\beta} \tau^3_{\gamma,\beta} \quad (3r_T r_V^2 N_o) \quad (8095)$$

$$\tau^3_{\gamma,\alpha} = \sum_{i \in O} W^1_{i,\alpha} Y^4_{i,\gamma} \quad (2r_T r_V N_o) \quad (8108)$$

$$\tau^5_{\gamma,\alpha} = \sum_{i \in O} W^1_{i,\alpha} Y^2_{i,\gamma} \quad (2r_T r_V N_o) \quad (8096)$$

$$\tau^4_{\gamma,\alpha,w} = \sum_{\delta \in A} \sum_{i \in O} {}^2D^2_{i,w} Y^{2,*}_{i,\gamma} \tau^3_{\delta,\alpha} \tau^0_{\delta,\gamma,w} \tau^2_{\delta,\alpha,i} \quad (5r_D r_T^2 r_V N_o) \quad (8109)$$

$$\tau^6_{\gamma,\alpha} = \sum_{a \in V} W^2_{a,\alpha} Y^3_{a,\gamma} \quad (2r_T r_V N_v) \quad (8097)$$

$$\tau^5_{\gamma,\alpha,w} = \sum_{\beta \in B} X_{\beta,\alpha} \tau^4_{\gamma,\beta,w} \quad (2r_D r_T r_V^2) \quad (8110)$$

$$\tau^7_{\gamma,\delta,i} = \sum_{\alpha \in B} \tau^5_{\gamma,\alpha} \tau^6_{\delta,\alpha} \tau^4_{\gamma,\alpha,i} \quad (3r_T^2 r_V N_o) \quad (8098)$$

$$\tau^6_{\gamma,\delta,w} = \sum_{a \in V} {}^2D^3_{a,w} Y^1_{a,\gamma} Y^{3,*}_{a,\delta} \quad (3r_D r_T^2 N_v) \quad (8111)$$

$$\tau^8_{\gamma,\delta,\epsilon} = \sum_{i \in O} Y^2_{i,\delta} Z_{\delta,\epsilon} \tau^7_{\gamma,\epsilon,i} \quad (3r_T^3 N_o) \quad (8099)$$

$$\tau^7_{\gamma,\alpha} = \sum_{i \in O} W^3_{i,\alpha} Y^2_{i,\gamma} \quad (2r_T r_V N_o) \quad (8112)$$

$$\tau^9_{\gamma,\delta,i} = \sum_{\epsilon \in A} Y^4_{i,\epsilon} \tau^8_{\gamma,\delta,\epsilon} \quad (2r_T^3 N_o) \quad (8100)$$

$$\tau^8_{\gamma,\alpha} = \sum_{a \in V} W^4_{a,\alpha} Y^3_{a,\gamma} \quad (2r_T r_V N_v) \quad (8113)$$

$$\tau^{10}_{\gamma,\delta,w} = \sum_{\epsilon \in A} \sum_{i \in O} {}^2D^4_{i,w} Y^{4,*}_{i,\delta} \tau^2_{\epsilon,\delta,w} \tau^9_{\gamma,\epsilon,i} \quad (4r_D r_T^3 N_o) \quad (8101)$$

$$\tau^9_{\gamma,\alpha,i} = \sum_{\delta \in A} Z_{\gamma,\delta} Y^4_{i,\delta} \tau^8_{\delta,\alpha} \quad (3r_T^2 r_V N_o) \quad (8114)$$

$$\tau^{11}_{\gamma,\delta,w} = \sum_{\epsilon \in A} Z_{\epsilon,\gamma} \tau^{10}_{\epsilon,\delta,w} \quad (2r_D r_T^3) \quad (8102)$$

$$\tau^{10}_{\gamma,\alpha,w} = \sum_{\delta \in A} \sum_{i \in O} {}^2D^4_{i,w} Y^{4,*}_{i,\gamma} \tau^7_{\delta,\alpha} \tau^6_{\delta,\gamma,w} \tau^9_{\delta,\alpha,i} \quad (5r_D r_T^2 r_V N_o) \quad (8115)$$

$${}^2R^z_{\gamma,\delta} \leftarrow \sum_{\epsilon \in A} \sum_{w \in D} \frac{1}{4} \tau^0_{\epsilon,\gamma,w} \tau^1_{\epsilon,\gamma,w} \tau^{11}_{\epsilon,\delta,w} \quad (3r_D r_T^3) \quad (8103)$$

$${}^2R^z_{\gamma,\delta} \leftarrow \sum_{\alpha \in B} \sum_{w \in D} \frac{1}{4} \tau^{10}_{\delta,\alpha,w} \tau^5_{\gamma,\alpha,w} \quad (2r_D r_T^2 r_V) \quad (8116)$$

Raw expression

$${}^2R^z_{\epsilon,\zeta} \leftarrow \sum_{i \in O} \sum_{j \in O} \sum_{k \in O} \sum_{l \in O} \sum_{a \in V} \sum_{b \in V} \sum_{c \in V} \sum_{d \in V} \frac{1}{4} Y^{1,*}_{a,\epsilon} Y^{2,*}_{i,\epsilon} Y^{3,*}_{b,\zeta} Y^{4,*}_{j,\zeta} {}^2D^{a,i,b,j} {}^2T_{b,k,a,l} {}^2T_{c,i,d,j} V_{k,d,l,c} \quad (8104)$$

Factorized expression

Raw expression

$${}^2R^z_{\epsilon,\zeta} \leftarrow \sum_{i \in O} \sum_{j \in O} \sum_{k \in O} \sum_{l \in O} \sum_{a \in V} \sum_{b \in V} \sum_{c \in V} \sum_{d \in V} \frac{1}{4} Y^{1,*}_{a,\epsilon} Y^{2,*}_{i,\epsilon} Y^{3,*}_{b,\zeta} Y^{4,*}_{j,\zeta} {}^2D^{a,i,b,j} {}^2T_{b,k,a,l} {}^2T_{c,j,d,i} V_{k,c,l,d} \quad (8117)$$

Factorized expression

$$\tau^0_{\gamma,\alpha} = \sum_{a \in V} W^2_{a,\alpha} Y^1_{a,\gamma} \quad (2r_T r_V N_v) \quad (8118)$$

$$\tau^1_{\gamma,\alpha,i} = \sum_{\beta \in B} W^1_{i,\beta} X_{\beta,\alpha} \tau^0_{\gamma,\beta} \quad (3r_T r_V^2 N_o) \quad (8119)$$

$$\tau^2_{\gamma,\alpha} = \sum_{a \in V} W^4_{a,\alpha} Y^3_{a,\gamma} \quad (2r_T r_V N_v) \quad (8120)$$

$$\tau^3_{\gamma,\alpha,i} = \sum_{\delta \in A} Z_{\gamma,\delta} Y^4_{i,\delta} \tau^2_{\delta,\alpha} \quad (3r_T^2 r_V N_o) \quad (8121)$$

$$\tau^4_{\gamma,i,j,k} = \sum_{\alpha \in B} W^3_{j,\alpha} \tau^1_{\gamma,\alpha,i} \tau^3_{\gamma,\alpha,k} \quad (3r_T r_V N_o^3) \quad (8122)$$

$$\tau^5_{i,j,k,l} = \sum_{\gamma \in A} Y^2_{k,\gamma} \tau^4_{\gamma,i,j,l} \quad (2r_T N_o^4) \quad (8123)$$

$$\tau^6_{\gamma,i,j,k} = \sum_{l \in O} Y^4_{l,\gamma} \tau^5_{i,l,j,k} \quad (2r_T N_o^4) \quad (8124)$$

$$\tau^7_{\gamma,\delta,w} = \sum_{a \in V} {}^2D^3_{a,w} Y^1_{a,\gamma} Y^{3,*}_{a,\delta} \quad (3r_D r_T^2 N_v) \quad (8125)$$

$$\tau^8_{\gamma,\delta,w,i} = \sum_{\epsilon \in A} Y^2_{i,\epsilon} Z_{\epsilon,\gamma} \tau^7_{\epsilon,\delta,w} \quad (3r_D r_T^3 N_o) \quad (8126)$$

$$\tau^9_{\gamma,\delta,w,i} = \sum_{j \in O} \sum_{k \in O} {}^2D^4_{j,w} Y^{4,*}_{j,\delta} \tau^6_{\gamma,k,j,i} \tau^8_{\gamma,\delta,w,k} \quad (4r_D r_T^2 N_o^3) \quad (8127)$$

$$\tau^{10}_{\gamma,\delta,w} = \sum_{a \in V} {}^2D^1_{a,w} Y^3_{a,\gamma} Y^{1,*}_{a,\delta} \quad (3r_D r_T^2 N_v) \quad (8128)$$

$${}^2R^z_{\gamma,\delta} \leftarrow \sum_{\epsilon \in A} \sum_{w \in D} \sum_{i \in O} \frac{1}{4} {}^2D^2_{i,w} Y^{2,*}_{i,\gamma} \tau^{10}_{\epsilon,\gamma,w} \tau^9_{\epsilon,\delta,w,i} \quad (4r_D r_T^2 N_o) \quad (8129)$$

Raw expression

$${}^2R^z_{\epsilon,\zeta} \leftarrow \sum_{i \in O} \sum_{j \in O} \sum_{k \in O} \sum_{l \in O} \sum_{a \in V} \sum_{b \in V} \sum_{c \in V} \sum_{d \in V} \frac{1}{4} Y^{1,*}_{a,\epsilon} Y^{2,*}_{i,\epsilon} Y^{3,*}_{b,\zeta} Y^{4,*}_{j,\zeta} {}^2D^{a,i,b,j} T_{b,k,d,i} {}^2T_{c,j,a,l} V_{l,d,k,c} \quad (8130)$$

Factorized expression

$$\tau^0_{\gamma,\delta,w} = \sum_{a \in V} {}^2D^3_{a,w} Y^1_{a,\gamma} Y^{3,*}_{a,\delta} \quad (3r_D r_T^2 N_v) \quad (8131)$$

$$\tau^1_{\gamma,\delta,w,i} = \sum_{\epsilon \in A} Y^2_{i,\epsilon} Z_{\epsilon,\gamma} \tau^0_{\epsilon,\delta,w} \quad (3r_D r_T^3 N_o) \quad (8132)$$

$$\tau^2_{\gamma,\alpha} = \sum_{a \in V} W^4_{a,\alpha} Y^1_{a,\gamma} \quad (2r_T r_V N_v) \quad (8133)$$

$$\tau^3_{\gamma,\alpha,i} = \sum_{\beta \in B} X_{\alpha,\beta} W^3_{i,\beta} \tau^2_{\gamma,\beta} \quad (3r_T r_V^2 N_o) \quad (8134)$$

$$\tau^4_{\gamma,\alpha} = \sum_{a \in V} W^2_{a,\alpha} Y^3_{a,\gamma} \quad (2r_T r_V N_v) \quad (8135)$$

$$\tau^5_{\gamma,\alpha,i} = \sum_{\delta \in A} Z_{\gamma,\delta} Y^4_{i,\delta} \tau^4_{\delta,\alpha} \quad (3r_T^2 r_V N_o) \quad (8136)$$

$$\tau^6_{\gamma,i,j,k} = \sum_{\alpha \in B} W^1_{i,\alpha} \tau^3_{\gamma,\alpha,j} \tau^5_{\gamma,\alpha,k} \quad (3r_T r_V N_o^3) \quad (8137)$$

$$\tau^7_{i,j,k,l} = \sum_{\gamma \in A} Y^2_{k,\gamma} \tau^6_{\gamma,i,j,l} \quad (2r_T N_o^4) \quad (8138)$$

$$\tau^8_{\gamma,i,j,k} = \sum_{l \in O} Y^4_{l,\gamma} \tau^7_{i,l,j,k} \quad (2r_T N_o^4) \quad (8139)$$

$$\tau^9_{\gamma,\delta,w,i} = \sum_{j \in O} \sum_{k \in O} {}^2D^4_{j,w} Y^{4,*}_{j,\delta} \tau^1_{\gamma,\delta,w,k} \tau^8_{\gamma,k,i,j} \quad (4r_D r_T^2 N_o^3) \quad (8140)$$

$$\tau^{10}_{\gamma,\delta,w} = \sum_{a \in V} {}^2D^1_{a,w} Y^3_{a,\gamma} Y^{1,*}_{a,\delta} \quad (3r_D r_T^2 N_v) \quad (8141)$$

$${}^2R^z_{\epsilon,\zeta} \leftarrow \sum_{\epsilon \in A} \sum_{w \in D} \sum_{i \in O} \frac{1}{4} {}^2D^2_{i,w} Y^{2,*}_{i,\gamma} \tau^{10}_{\epsilon,\gamma,w} \tau^9_{\epsilon,\delta,w,i} \quad (4r_D r_T^2 N_o) \quad (8142)$$

Raw expression

$${}^2R^z_{\epsilon,\zeta} \leftarrow \sum_{i \in O} \sum_{j \in O} \sum_{k \in O} \sum_{l \in O} \sum_{a \in V} \sum_{b \in V} \sum_{c \in V} \sum_{d \in V} \frac{1}{4} Y^{1,*}_{a,\epsilon} Y^{2,*}_{i,\epsilon} Y^{3,*}_{b,\zeta} Y^{4,*}_{j,\zeta} {}^2D^{a,i,b,j} T_{b,k,d,j} {}^2T_{c,i,a,l} V_{l,c,k,d} \quad (8143)$$

Factorized expression

$$\tau^0_{\gamma,\delta,w} = \sum_{a \in V} {}^2D^1_{a,w} Y^3_{a,\gamma} Y^{1,*}_{a,\delta} \quad (3r_D r_T^2 N_v) \quad (8144)$$

$$\tau^1_{\gamma,\delta,w} = \sum_{i \in O} {}^2D^2_{i,w} Y^4_{i,\gamma} Y^{2,*}_{i,\delta} \quad (3r_D r_T^2 N_o) \quad (8145)$$

$$\tau^2_{\gamma,\delta,w} = \sum_{i \in O} {}^2D^4_{i,w} Y^2_{i,\gamma} Y^{4,*}_{i,\delta} \quad (3r_D r_T^2 N_o) \quad (8146)$$

$$\tau^3_{\gamma,\alpha} = \sum_{a \in V} W^2_{a,\alpha} Y^3_{a,\gamma} \quad (2r_T r_V N_v) \quad (8147)$$

$$\tau^4_{\gamma,\alpha,i} = \sum_{\beta \in B} W^1_{i,\beta} X_{\beta,\alpha} \tau^3_{\gamma,\beta} \quad (3r_T r_V^2 N_o) \quad (8148)$$

$$\tau^5_{\gamma,\alpha} = \sum_{i \in O} W^3_{i,\alpha} Y^4_{i,\gamma} \quad (2r_T r_V N_o) \quad (8149)$$

$$\tau^6_{\gamma,\alpha} = \sum_{\delta \in A} \sum_{i \in O} Y^2_{i,\gamma} Z_{\gamma,\delta} \tau^5_{\delta,\alpha} \tau^4_{\delta,\alpha,i} \quad (4r_T^2 r_V N_o) \quad (8150)$$

$$\tau^7_{\gamma,a} = \sum_{\alpha \in B} W^4_{a,\alpha} \tau^6_{\gamma,\alpha} \quad (2r_T r_V N_v) \quad (8151)$$

$$\tau^8_{\gamma,\delta} = \sum_{a \in V} Y^1_{a,\gamma} \tau^7_{\delta,a} \quad (2r_T^2 N_v) \quad (8152)$$

$$\tau^9_{\gamma,a} = \sum_{\delta \in A} Y^1_{a,\delta} \tau^8_{\gamma,\delta} \quad (2r_T^2 N_v) \quad (8153)$$

$$\tau^{10}_{\gamma,\delta,w} = \sum_{a \in V} {}^2D^3_{a,w} Y^{3,*}_{a,\delta} \tau^9_{\gamma,a} \quad (3r_D r_T^2 N_v) \quad (8154)$$

$$\tau^{11}_{\gamma,\delta,w} = \sum_{\epsilon \in A} Z_{\epsilon,\gamma} \tau^{10}_{\epsilon,\delta,w} \tau^2_{\epsilon,\delta,w} \quad (3r_D r_T^3) \quad (8155)$$

$${}^2R^z_{\gamma,\delta} \leftarrow \sum_{\epsilon \in A} \sum_{w \in D} \frac{1}{4} \tau^0_{\epsilon,\gamma,w} \tau^1_{\epsilon,\gamma,w} \tau^{11}_{\epsilon,\delta,w} \quad (3r_D r_T^3) \quad (8156)$$

Raw expression

$${}^2R^z_{\epsilon,\zeta} \leftarrow \sum_{i \in O} \sum_{j \in O} \sum_{k \in O} \sum_{l \in O} \sum_{a \in V} \sum_{b \in V} \sum_{c \in V} \sum_{d \in V} \frac{1}{4} Y^{1,*}_{a,\epsilon} Y^{2,*}_{i,\epsilon} Y^{3,*}_{b,\zeta} Y^{4,*}_{j,\zeta} {}^2D^{a,i,b,j}_{a,\gamma} {}^2T_{b,k,d,l} {}^2T_{c,j,a,i} V_{k,d,l,c} \quad (8157)$$

Factorized expression

$$\tau^0_{\gamma,\delta,w} = \sum_{a \in V} {}^2D^1_{a,w} Y^3_{a,\gamma} Y^{1,*}_{a,\delta} \quad (3r_D r_T^2 N_v) \quad (8158)$$

$$\tau^1_{\gamma,\delta,w} = \sum_{i \in O} {}^2D^2_{i,w} Y^4_{i,\gamma} Y^{2,*}_{i,\delta} \quad (3r_D r_T^2 N_o) \quad (8159)$$

$$\tau^2_{\gamma,\delta,w} = \sum_{\epsilon \in A} Z_{\gamma,\epsilon} \tau^0_{\epsilon,\delta,w} \tau^1_{\epsilon,\delta,w} \quad (3r_D r_T^3) \quad (8160)$$

$$\tau^3_{\gamma,\alpha} = \sum_{a \in V} W^2_{a,\alpha} Y^3_{a,\gamma} \quad (2r_T r_V N_v) \quad (8161)$$

$$\tau^4_{\gamma,\alpha,i} = \sum_{\beta \in B} W^1_{i,\beta} X_{\beta,\alpha} \tau^3_{\gamma,\beta} \quad (3r_T r_V^2 N_o) \quad (8162)$$

$$\tau^5_{\gamma,\alpha} = \sum_{i \in O} W^3_{i,\alpha} Y^4_{i,\gamma} \quad (2r_T r_V N_o) \quad (8163)$$

$$\tau^6_{\gamma,\alpha} = \sum_{a \in V} W^4_{a,\alpha} Y^1_{a,\gamma} \quad (2r_T r_V N_v) \quad (8164)$$

$$\tau^7_{\gamma,\delta,i} = \sum_{\alpha \in B} \tau^5_{\delta,\alpha} \tau^6_{\gamma,\alpha} \tau^4_{\delta,\alpha,i} \quad (3r_T^2 r_V N_o) \quad (8165)$$

$$\tau^8_{\gamma,i} = \sum_{\delta \in A} Z_{\gamma,\delta} \tau^7_{\gamma,\delta,i} \quad (2r_T^2 N_o) \quad (8166)$$

$$\tau^9_{i,j} = \sum_{\gamma \in A} Y^2_{j,\gamma} \tau^8_{\gamma,i} \quad (2r_T N_o^2) \quad (8167)$$

$$\tau^{10}_{\gamma,i} = \sum_{j \in O} Y^2_{j,\gamma} \tau^9_{j,i} \quad (2r_T N_o^2) \quad (8168)$$

$$\tau^{11}_{\gamma,\delta,w} = \sum_{i \in O} {}^2D^4_{i,w} Y^{4,*}_{i,\delta} \tau^{10}_{\gamma,i} \quad (3r_D r_T^2 N_o) \quad (8169)$$

$$\tau^{12}_{\gamma,\delta,w} = \sum_{a \in V} {}^2D^3_{a,w} Y^1_{a,\gamma} Y^{3,*}_{a,\delta} \quad (3r_D r_T^2 N_v) \quad (8170)$$



$${}^2R^z_{\gamma,\delta} \leftarrow \sum_{\epsilon \in A} \sum_{w \in D} \frac{1}{4} \tau^{11}_{\epsilon,\delta,w} \tau^{12}_{\epsilon,\delta,w} \tau^2_{\epsilon,\gamma,w} \quad (3r_D r_T^3) \quad (8171)$$

Raw expression

$${}^2R^z_{\epsilon,\zeta} \leftarrow \sum_{i \in O} \sum_{j \in O} \sum_{k \in O} \sum_{l \in O} \sum_{a \in V} \sum_{b \in V} \sum_{c \in V} \sum_{d \in V} \frac{1}{4} Y^{1,*}_{a,\epsilon} Y^{2,*}_{i,\epsilon} Y^{3,*}_{b,\zeta} Y^{4,*}_{j,\zeta} {}^2D^{a,i,b,j} {}^2T_{b,l,d,j} {}^2T_{c,k,a,i} V_{k,d,l,c} \quad (8172)$$

Factorized expression

$$\tau^0_{\gamma,\alpha} = \sum_{a \in V} W^2_{a,\alpha} Y^3_{a,\gamma} \quad (2r_T r_V N_v) \quad (8173)$$

$$\tau^1_{\gamma,\alpha,i} = \sum_{\beta \in B} W^1_{i,\beta} X_{\beta,\alpha} \tau^0_{\gamma,\beta} \quad (3r_T r_V^2 N_o) \quad (8174)$$

$$\tau^2_{\gamma,\delta,\alpha} = \sum_{i \in O} Y^4_{i,\delta} \tau^1_{\gamma,\alpha,i} \quad (2r_T^2 r_V N_o) \quad (8175)$$

$$\tau^3_{\gamma,\alpha} = \sum_{a \in V} W^4_{a,\alpha} Y^1_{a,\gamma} \quad (2r_T r_V N_v) \quad (8176)$$

$$\tau^4_{\gamma,\alpha,i} = \sum_{\delta \in A} Y^2_{i,\delta} Z_{\delta,\gamma} \tau^3_{\delta,\alpha} \quad (3r_T^2 r_V N_o) \quad (8177)$$

$$\tau^5_{\gamma,\delta,\alpha,w} = \sum_{i \in O} {}^2D^4_{i,w} Y^{4,*}_{i,\delta} \tau^4_{\gamma,\alpha,i} \quad (3r_D r_T^2 r_V N_o) \quad (8178)$$

$$\tau^6_{\gamma,\delta,w} = \sum_{a \in V} {}^2D^3_{a,w} Y^1_{a,\gamma} Y^{3,*}_{a,\delta} \quad (3r_D r_T^2 N_v) \quad (8179)$$

$$\tau^7_{\gamma,\delta,w,i} = \sum_{\epsilon \in A} Y^2_{i,\epsilon} Z_{\epsilon,\gamma} \tau^6_{\epsilon,\delta,w} \quad (3r_D r_T^3 N_o) \quad (8180)$$

$$\tau^8_{\gamma,\delta,\alpha,w} = \sum_{i \in O} W^3_{i,\alpha} \tau^7_{\gamma,\delta,w,i} \quad (2r_D r_T^2 r_V N_o) \quad (8181)$$

$$\tau^9_{\gamma,\delta,\epsilon,w} = \sum_{\alpha \in B} \tau^2_{\gamma,\delta,\alpha} \tau^5_{\delta,\epsilon,\alpha,w} \tau^8_{\gamma,\epsilon,\alpha,w} \quad (3r_D r_T^3 r_V) \quad (8182)$$

$$\tau^{10}_{\gamma,\delta,w,i} = \sum_{\epsilon \in A} {}^2D^2_{i,w} Y^4_{i,\epsilon} \tau^9_{\epsilon,\gamma,\delta,w} \quad (3r_D r_T^3 N_o) \quad (8183)$$

$$\tau^{11}_{\gamma,\delta,w} = \sum_{a \in V} {}^2D^1_{a,w} Y^3_{a,\gamma} Y^{1,*}_{a,\delta} \quad (3r_D r_T^2 N_v) \quad (8184)$$

$$\tau^{12}_{\gamma,\delta,i} = \sum_{\epsilon \in A} \sum_{w \in D} \tau^{11}_{\epsilon,\gamma,w} \tau^{10}_{\epsilon,\delta,w,i} \quad (2r_D r_T^3 N_o) \quad (8185)$$

$${}^2R^z_{\gamma,\delta} \leftarrow \sum_{i \in O} \frac{1}{4} Y^{2,*}_{i,\gamma} \tau^{12}_{\gamma,\delta,i} \quad (2r_T^2 N_o) \quad (8186)$$

Raw expression

$${}^2R^z_{\epsilon,\zeta} \leftarrow \sum_{i \in O} \sum_{j \in O} \sum_{k \in O} \sum_{l \in O} \sum_{a \in V} \sum_{b \in V} \sum_{c \in V} \sum_{d \in V} \frac{1}{4} Y^{1,*}_{a,\epsilon} Y^{2,*}_{i,\epsilon} Y^{3,*}_{b,\zeta} Y^{4,*}_{j,\zeta} {}^2D^{a,i,b,j} {}^2T_{c,i,a,k} {}^2T_{d,j,b,l} V_{k,c,l,d} \quad (8187)$$

Factorized expression

$$\tau^0_{\gamma,\delta,w} = \sum_{a \in V} {}^2D^1_{a,w} Y^3_{a,\gamma} Y^{1,*}_{a,\delta} \quad (3r_D r_T^2 N_v) \quad (8188)$$

$$\tau^1_{\gamma,\alpha} = \sum_{a \in V} W^2_{a,\alpha} Y^1_{a,\gamma} \quad (2r_T r_V N_v) \quad (8189)$$

$$\tau^2_{\gamma,\alpha,i} = \sum_{\delta \in A} Y^2_{i,\delta} Z_{\delta,\gamma} \tau^1_{\delta,\alpha} \quad (3r_T^2 r_V N_o) \quad (8190)$$

$$\tau^3_{\gamma,\alpha} = \sum_{i \in O} W^1_{i,\alpha} Y^4_{i,\gamma} \quad (2r_T r_V N_o) \quad (8191)$$

$$\tau^4_{\gamma,\alpha,w} = \sum_{\delta \in A} \sum_{i \in O} {}^2D^2_{i,w} Y^{2,*}_{i,\gamma} \tau^3_{\delta,\alpha} \tau^0_{\delta,\gamma,w} \tau^2_{\delta,\alpha,i} \quad (5r_D r_T^2 r_V N_o) \quad (8192)$$

$$\tau^5_{\gamma,\alpha,w} = \sum_{\beta \in B} X_{\beta,\alpha} \tau^4_{\gamma,\beta,w} \quad (2r_D r_T r_V^2) \quad (8193)$$

$$\tau^6_{\gamma,\delta,w} = \sum_{a \in V} {}^2D^3_{a,w} Y^3_{a,\gamma} Y^{3,*}_{a,\delta} \quad (3r_D r_T^2 N_v) \quad (8194)$$

$$\tau^7_{\gamma,\alpha} = \sum_{a \in V} W^4_{a,\alpha} Y^1_{a,\gamma} \quad (2r_T r_V N_v) \quad (8195)$$

$$\tau^8_{\gamma,\alpha,i} = \sum_{\delta \in A} Y^2_{i,\delta} Z_{\delta,\gamma} \tau^7_{\delta,\alpha} \quad (3r_T^2 r_V N_o) \quad (8196)$$

$$\tau_{\gamma,\alpha}^9 = \sum_{i \in O} W_{i,\alpha}^3 Y_{i,\gamma}^4 \quad (2r_T r_V N_o) \quad (8197)$$

$$\tau_{\gamma,\delta,\epsilon,w}^9 = \sum_{\alpha \in B} \tau_{\gamma,\delta,\alpha}^2 \tau_{\delta,\epsilon,\alpha,w}^5 \tau_{\gamma,\epsilon,\alpha,w}^8 \quad (3r_D r_T^3 r_V) \quad (8210)$$

$$\tau_{\gamma,\alpha,w}^{10} = \sum_{\delta \in A} \sum_{i \in O} {}^2D_{i,w}^4 Y_{i,\gamma}^{4,*} \tau_{\delta,\alpha}^9 \tau_{\delta,\gamma,w}^6 \tau_{\delta,\alpha,i}^8 \quad (5r_D r_T^2 r_V N_o) \quad (8198)$$

$$\tau_{\gamma,\delta,w,i}^{10} = \sum_{\epsilon \in A} {}^2D_{i,w}^2 Y_{i,\epsilon}^2 \tau_{\epsilon,\gamma,\delta,w}^9 \quad (3r_D r_T^3 N_o) \quad (8211)$$

$${}^2R_{\gamma,\delta}^z \leftarrow \sum_{\alpha \in B} \sum_{w \in D} \frac{1}{4} \tau_{\delta,\alpha,w}^{10} \tau_{\gamma,\alpha,w}^5 \quad (2r_D r_T^2 r_V) \quad (8199)$$

$$\tau_{\gamma,\delta,w}^{11} = \sum_{a \in V} {}^2D_{a,w}^1 Y_{a,\gamma}^3 Y_{a,\delta}^{1,*} \quad (3r_D r_T^2 N_v) \quad (8212)$$

Raw expression

$${}^2R_{\epsilon,\zeta}^z \leftarrow \sum_{i \in O} \sum_{j \in O} \sum_{k \in O} \sum_{l \in O} \sum_{a \in V} \sum_{b \in V} \sum_{c \in V} \sum_{d \in V} \frac{1}{4} Y_{a,\epsilon}^{1,*} Y_{i,\epsilon}^{2,*} Y_{b,\zeta}^{3,*} Y_{j,\zeta}^{4,*} {}^2D_{a,i,b,j} {}^2T_{c,i,a,l} {}^2T_{d,k,b,j} V_{l,d,k,c} \quad (8200)$$

$$\tau_{\gamma,\delta,i}^{12} = \sum_{\epsilon \in A} \sum_{w \in D} \tau_{\epsilon,\gamma,w}^{11} \tau_{\epsilon,\delta,w,i}^{10} \quad (2r_D r_T^3 N_o) \quad (8213)$$

Factorized expression

$${}^2R_{\gamma,\delta}^z \leftarrow \sum_{i \in O} \frac{1}{4} Y_{i,\gamma}^{2,*} \tau_{\gamma,\delta,i}^{12} \quad (2r_T^2 N_o) \quad (8214)$$

$$\tau_{\gamma,\alpha}^0 = \sum_{a \in V} W_{a,\alpha}^2 Y_{a,\gamma}^1 \quad (2r_T r_V N_v) \quad (8201)$$

Raw expression

$$\tau_{\gamma,\alpha,i}^1 = \sum_{\beta \in B} W_{i,\beta}^1 X_{\beta,\alpha} \tau_{\gamma,\beta}^0 \quad (3r_T r_V^2 N_o) \quad (8202)$$

$${}^2R_{\epsilon,\zeta}^z \leftarrow \sum_{i \in O} \sum_{j \in O} \sum_{k \in O} \sum_{l \in O} \sum_{a \in V} \sum_{b \in V} \sum_{c \in V} \sum_{d \in V} \frac{1}{4} Y_{a,\epsilon}^{1,*} Y_{i,\epsilon}^{2,*} Y_{b,\zeta}^{3,*} Y_{j,\zeta}^{4,*} {}^2D_{a,i,b,j} {}^2T_{c,i,b,j} {}^2T_{d,k,a,l} V_{k,c,l,d} \quad (8215)$$

$$\tau_{\gamma,\delta,\alpha}^2 = \sum_{i \in O} Y_{i,\delta}^4 \tau_{\gamma,\alpha,i}^1 \quad (2r_T^2 r_V N_o) \quad (8203)$$

Factorized expression

$$\tau_{\gamma,\alpha}^3 = \sum_{a \in V} W_{a,\alpha}^4 Y_{a,\gamma}^1 \quad (2r_T r_V N_v) \quad (8204)$$

$$\tau_{\gamma,\delta,w}^0 = \sum_{i \in O} {}^2D_{i,w}^2 Y_{i,\gamma}^2 Y_{i,\delta}^{2,*} \quad (3r_D r_T^2 N_o) \quad (8216)$$

$$\tau_{\gamma,\alpha,i}^4 = \sum_{\delta \in A} Y_{i,\delta}^2 Z_{\delta,\gamma} \tau_{\delta,\alpha}^3 \quad (3r_T^2 r_V N_o) \quad (8205)$$

$$\tau_{\gamma,\alpha}^1 = \sum_{a \in V} W_{a,\alpha}^4 Y_{a,\gamma}^1 \quad (2r_T r_V N_v) \quad (8217)$$

$$\tau_{\gamma,\delta,\alpha,w}^5 = \sum_{i \in O} {}^2D_{i,w}^4 Y_{i,\delta}^{4,*} \tau_{\gamma,\alpha,i}^4 \quad (3r_D r_T^2 r_V N_o) \quad (8206)$$

$$\tau_{\gamma,\alpha,i}^2 = \sum_{\beta \in B} X_{\alpha,\beta} W_{i,\beta}^3 \tau_{\gamma,\beta}^1 \quad (3r_T r_V^2 N_o) \quad (8218)$$

$$\tau_{\gamma,\delta,w}^6 = \sum_{a \in V} {}^2D_{a,w}^3 Y_{a,\gamma}^3 Y_{a,\delta}^{3,*} \quad (3r_D r_T^2 N_v) \quad (8207)$$

$$\tau_{\gamma,\alpha}^3 = \sum_{i \in O} W_{i,\alpha}^1 Y_{i,\gamma}^2 \quad (2r_T r_V N_o) \quad (8219)$$

$$\tau_{\gamma,\delta,w,i}^7 = \sum_{\epsilon \in A} Z_{\gamma,\epsilon} Y_{i,\epsilon}^4 \tau_{\epsilon,\delta,w}^6 \quad (3r_D r_T^3 N_o) \quad (8208)$$

$$\tau_{\gamma,\alpha}^4 = \sum_{\delta \in A} \sum_{i \in O} Z_{\delta,\gamma} Y_{i,\gamma}^4 \tau_{\delta,\alpha}^3 \tau_{\delta,\alpha,i}^2 \quad (4r_T^2 r_V N_o) \quad (8220)$$

$$\tau_{\gamma,\delta,\alpha,w}^8 = \sum_{i \in O} W_{i,\alpha}^3 \tau_{\gamma,\delta,w,i}^7 \quad (2r_D r_T^2 r_V N_o) \quad (8209)$$

$$\tau_{\gamma,\alpha}^5 = \sum_{\alpha \in B} W_{a,\alpha}^2 \tau_{\gamma,\alpha}^4 \quad (2r_T r_V N_v) \quad (8221)$$

$$\tau^6_{a,b} = \sum_{\gamma \in A} Y^3_{b,\gamma} \tau^5_{\gamma,a} \quad (2r_T N_v^2) \quad (8222)$$

$$\tau^7_{\gamma,a} = \sum_{b \in V} Y^1_{b,\gamma} \tau^6_{b,a} \quad (2r_T N_v^2) \quad (8223)$$

$$\tau^8_{\gamma,\delta,w} = \sum_{a \in V} {}^2D^1_{a,w} Y^{1,*}_{a,\delta} \tau^7_{\gamma,a} \quad (3r_D r_T^2 N_v) \quad (8224)$$

$$\tau^9_{\gamma,\delta,w} = \sum_{a \in V} {}^2D^3_{a,w} Y^3_{a,\gamma} Y^{3,*}_{a,\delta} \quad (3r_D r_T^2 N_v) \quad (8225)$$

$$\tau^{10}_{\gamma,\delta,w} = \sum_{i \in O} {}^2D^4_{i,w} Y^4_{i,\gamma} Y^{4,*}_{i,\delta} \quad (3r_D r_T^2 N_o) \quad (8226)$$

$$\tau^{11}_{\gamma,\delta,w} = \sum_{\epsilon \in A} Z_{\gamma,\epsilon} \tau^{10}_{\epsilon,\delta,w} \tau^9_{\epsilon,\delta,w} \quad (3r_D r_T^3) \quad (8227)$$

$${}^2R^z_{\gamma,\delta} \leftarrow \sum_{\epsilon \in A} \sum_{w \in D} \frac{1}{4} \tau^0_{\epsilon,\gamma,w} \tau^{11}_{\epsilon,\delta,w} \tau^8_{\epsilon,\gamma,w} \quad (3r_D r_T^3) \quad (8228)$$

Raw expression

$${}^2R^z_{\epsilon,\zeta} \leftarrow \sum_{i \in O} \sum_{j \in O} \sum_{k \in O} \sum_{l \in O} \sum_{a \in V} \sum_{b \in V} \sum_{c \in V} \sum_{d \in V} \frac{1}{4} Y^{1,*}_{a,\epsilon} Y^{2,*}_{i,\epsilon} Y^{3,*}_{b,\zeta} Y^{4,*}_{j,\zeta} {}^2D^{a,i,b,j} {}^2T_{c,i,b,l} {}^2T_{d,j,a,k} V_{k,c,l,d} \quad (8229)$$

Factorized expression

$$\tau^0_{\gamma,\delta,w} = \sum_{a \in V} {}^2D^1_{a,w} Y^3_{a,\gamma} Y^{1,*}_{a,\delta} \quad (3r_D r_T^2 N_v) \quad (8230)$$

$$\tau^1_{\gamma,\delta,w} = \sum_{i \in O} {}^2D^2_{i,w} Y^4_{i,\gamma} Y^{2,*}_{i,\delta} \quad (3r_D r_T^2 N_o) \quad (8231)$$

$$\tau^2_{\gamma,\delta,w} = \sum_{\epsilon \in A} Z_{\gamma,\epsilon} \tau^0_{\epsilon,\delta,w} \tau^1_{\epsilon,\delta,w} \quad (3r_D r_T^3) \quad (8232)$$

$$\tau^3_{\gamma,\delta,w} = \sum_{i \in O} {}^2D^4_{i,w} Y^2_{i,\gamma} Y^{4,*}_{i,\delta} \quad (3r_D r_T^2 N_o) \quad (8233)$$

$$\tau^4_{\gamma,\alpha} = \sum_{a \in V} W^4_{a,\alpha} Y^1_{a,\gamma} \quad (2r_T r_V N_v) \quad (8234)$$

$$\tau^5_{\gamma,\alpha,i} = \sum_{\beta \in B} X_{\alpha,\beta} W^3_{i,\beta} \tau^4_{\gamma,\beta} \quad (3r_T r_V^2 N_o) \quad (8235)$$

$$\tau^6_{\gamma,\alpha} = \sum_{i \in O} W^1_{i,\alpha} Y^2_{i,\gamma} \quad (2r_T r_V N_o) \quad (8236)$$

$$\tau^7_{\gamma,\alpha} = \sum_{\delta \in A} \sum_{i \in O} Z_{\delta,\gamma} Y^4_{i,\gamma} \tau^6_{\delta,\alpha} \tau^5_{\delta,\alpha,i} \quad (4r_T^2 r_V N_o) \quad (8237)$$

$$\tau^8_{\gamma,a} = \sum_{\alpha \in B} W^2_{a,\alpha} \tau^7_{\gamma,\alpha} \quad (2r_T r_V N_v) \quad (8238)$$

$$\tau^9_{a,b} = \sum_{\gamma \in A} Y^3_{b,\gamma} \tau^8_{\gamma,a} \quad (2r_T N_v^2) \quad (8239)$$

$$\tau^{10}_{\gamma,a} = \sum_{b \in V} Y^1_{b,\gamma} \tau^9_{b,a} \quad (2r_T N_v^2) \quad (8240)$$

$$\tau^{11}_{\gamma,\delta,w} = \sum_{a \in V} {}^2D^3_{a,w} Y^{3,*}_{a,\delta} \tau^{10}_{\gamma,a} \quad (3r_D r_T^2 N_v) \quad (8241)$$

$${}^2R^z_{\gamma,\delta} \leftarrow \sum_{\epsilon \in A} \sum_{w \in D} \frac{1}{4} \tau^{11}_{\epsilon,\delta,w} \tau^2_{\epsilon,\gamma,w} \tau^3_{\epsilon,\delta,w} \quad (3r_D r_T^3) \quad (8242)$$

Raw expression

$${}^2R^z_{\epsilon,\zeta} \leftarrow \sum_{i \in O} \sum_{j \in O} \sum_{k \in O} \sum_{l \in O} \sum_{a \in V} \sum_{b \in V} \sum_{c \in V} \sum_{d \in V} \frac{1}{4} Y^{1,*}_{a,\epsilon} Y^{2,*}_{i,\epsilon} Y^{3,*}_{b,\zeta} Y^{4,*}_{j,\zeta} {}^2D^{a,i,b,j} {}^2T_{c,j,a,i} {}^2T_{d,k,b,l} V_{k,c,l,d} \quad (8243)$$

Factorized expression

$$\tau^0_{\gamma,\delta,w} = \sum_{a \in V} {}^2D^1_{a,w} Y^3_{a,\gamma} Y^{1,*}_{a,\delta} \quad (3r_D r_T^2 N_v) \quad (8244)$$

$$\tau^1_{\gamma,\delta,w} = \sum_{i \in O} {}^2D^2_{i,w} Y^4_{i,\gamma} Y^{2,*}_{i,\delta} \quad (3r_D r_T^2 N_o) \quad (8245)$$

$$\tau^2_{\gamma,\delta,w} = \sum_{a \in V} {}^2D^3_{a,w} Y^3_{a,\gamma} Y^{3,*}_{a,\delta} \quad (3r_D r_T^2 N_v) \quad (8246)$$

$$\tau^3_{\gamma,\alpha} = \sum_{a \in V} W^4_{a,\alpha} Y^1_{a,\gamma} \quad (2r_T r_V N_v) \quad (8247)$$

$$\tau_{\gamma,\alpha,i}^4 = \sum_{\beta \in B} X_{\alpha,\beta} W_{i,\beta}^3 \tau_{\gamma,\beta}^3 \quad (3r_T r_V^2 N_o) \quad (8248)$$

$$\tau_{\gamma,\alpha}^3 = \sum_{i \in O} W_{i,\alpha}^3 Y_{i,\gamma}^2 \quad (2r_T r_V N_o) \quad (8261)$$

$$\tau_{\gamma,\alpha}^5 = \sum_{i \in O} W_{i,\alpha}^1 Y_{i,\gamma}^2 \quad (2r_T r_V N_o) \quad (8249)$$

$$\tau_{\gamma,\alpha}^4 = \sum_{a \in V} W_{a,\alpha}^4 Y_{a,\gamma}^1 \quad (2r_T r_V N_v) \quad (8262)$$

$$\tau_{\gamma,\alpha}^6 = \sum_{a \in V} W_{a,\alpha}^2 Y_{a,\gamma}^1 \quad (2r_T r_V N_v) \quad (8250)$$

$$\tau_{\gamma,\delta,i}^5 = \sum_{\alpha \in B} \tau_{\gamma,\alpha}^3 \tau_{\delta,\alpha}^4 \tau_{\gamma,\alpha,i}^2 \quad (3r_T^2 r_V N_o) \quad (8263)$$

$$\tau_{\gamma,\delta,i}^7 = \sum_{\alpha \in B} \tau_{\gamma,\alpha}^5 \tau_{\delta,\alpha}^6 \tau_{\gamma,\alpha,i}^4 \quad (3r_T^2 r_V N_o) \quad (8251)$$

$$\tau_{\gamma,\delta,\epsilon}^6 = \sum_{i \in O} Z_{\delta,\epsilon} Y_{i,\epsilon}^4 \tau_{\gamma,\delta,i}^5 \quad (3r_T^3 N_o) \quad (8264)$$

$$\tau_{\gamma,\delta,\epsilon}^8 = \sum_{i \in O} Z_{\delta,\epsilon} Y_{i,\epsilon}^4 \tau_{\gamma,\delta,i}^7 \quad (3r_T^3 N_o) \quad (8252)$$

$$\tau_{\gamma,\delta,i}^7 = \sum_{\epsilon \in A} Y_{i,\epsilon}^2 \tau_{\gamma,\epsilon,\delta}^6 \quad (2r_T^3 N_o) \quad (8265)$$

$$\tau_{\gamma,\delta,i}^9 = \sum_{\epsilon \in A} Y_{i,\epsilon}^2 \tau_{\gamma,\epsilon,\delta}^8 \quad (2r_T^3 N_o) \quad (8253)$$

$$\tau_{\gamma,\delta,w}^8 = \sum_{\epsilon \in A} \sum_{i \in O} {}^2D_{i,w}^2 Y_{i,\delta}^{2,*} \tau_{\epsilon,\delta,w}^0 \tau_{\gamma,\epsilon,i}^7 \quad (4r_D r_T^3 N_o) \quad (8266)$$

$$\tau_{\gamma,\delta,w}^{10} = \sum_{\epsilon \in A} \sum_{i \in O} {}^2D_{i,w}^4 Y_{i,\delta}^{4,*} \tau_{\epsilon,\delta,w}^2 \tau_{\gamma,\epsilon,i}^9 \quad (4r_D r_T^3 N_o) \quad (8254)$$

$$\tau_{\gamma,\delta,w}^9 = \sum_{a \in V} {}^2D_{a,w}^3 Y_{a,\gamma}^3 Y_{a,\delta}^{3,*} \quad (3r_D r_T^2 N_v) \quad (8267)$$

$$\tau_{\gamma,\delta,w}^{11} = \sum_{\epsilon \in A} Z_{\epsilon,\gamma} \tau_{\epsilon,\delta,w}^{10} \quad (2r_D r_T^3) \quad (8255)$$

$$\tau_{\gamma,\delta,w}^{10} = \sum_{i \in O} {}^2D_{i,w}^4 Y_{i,\gamma}^4 Y_{i,\delta}^{4,*} \quad (3r_D r_T^2 N_o) \quad (8268)$$

$${}^2R_{\gamma,\delta}^z \leftarrow \sum_{\epsilon \in A} \sum_{w \in D} \frac{1}{4} \tau_{\epsilon,\gamma,w}^0 \tau_{\epsilon,\gamma,w}^1 \tau_{\epsilon,\delta,w}^{11} \quad (3r_D r_T^3) \quad (8256)$$

$$\tau_{\gamma,\delta,w}^{11} = \sum_{\epsilon \in A} Z_{\gamma,\epsilon} \tau_{\epsilon,\delta,w}^{10} \tau_{\epsilon,\delta,w}^9 \quad (3r_D r_T^3) \quad (8269)$$

Raw expression

$${}^2R_{\epsilon,\zeta}^z \leftarrow \sum_{i \in O} \sum_{j \in O} \sum_{k \in O} \sum_{l \in O} \sum_{a \in V} \sum_{b \in V} \sum_{c \in V} \sum_{d \in V} \frac{1}{4} Y_{a,\epsilon}^{1,*} Y_{i,\epsilon}^{2,*} Y_{b,\zeta}^{3,*} Y_{j,\zeta}^{4,*} {}^2D_{a,i,b,j} {}^2T_{c,j,b,l} {}^2T_{d,k,a,i} V_{k,c,l,d} \quad (8257)$$

Factorized expression

$$\tau_{\gamma,\delta,w}^0 = \sum_{a \in V} {}^2D_{a,w}^1 Y_{a,\gamma}^3 Y_{a,\delta}^{1,*} \quad (3r_D r_T^2 N_v) \quad (8258)$$

$${}^2R_{\gamma,\delta}^z \leftarrow \sum_{\epsilon \in A} \sum_{w \in D} \frac{1}{4} \tau_{\epsilon,\delta,w}^{11} \tau_{\epsilon,\delta,w}^8 \tau_{\epsilon,\gamma,w}^8 \quad (2r_D r_T^3) \quad (8270)$$

## X. THC-RCCSD DOUBLES ( $Y^3$ FACTOR) EQUATION

Here expressions for a THC-RCCSD doubles residual, projected against all factors except  $Y^3$ , are given along with their cost

### A. Contributions from $H$

Raw expression

$$\tau_{\gamma,\alpha}^1 = \sum_{a \in V} W_{a,\alpha}^2 Y_{a,\gamma}^1 \quad (2r_T r_V N_v) \quad (8259)$$

$$\tau_{\gamma,\alpha,i}^2 = \sum_{\beta \in B} W_{i,\beta}^1 X_{\beta,\alpha} \tau_{\gamma,\beta}^1 \quad (3r_T r_V^2 N_o) \quad (8260)$$

$${}^2R_{b,\zeta}^3 \leftarrow \sum_{\gamma \in A} \sum_{i \in O} \sum_{j \in O} \sum_{a \in V} Y_{a,\gamma}^{1,*} Y_{i,\gamma}^{2,*} Z_{\gamma,\zeta}^* Y_{j,\zeta}^{4,*} {}^2D_{a,i,b,j} V_{a,i,b,j} \quad (8271)$$

Factorized expression

$$\tau^0_{\gamma,\alpha,w} = \sum_{i \in O} {}^2D^4_{i,w} W^4_{i,\alpha} Y^{4,*}_{i,\gamma} \quad (3r_D r_T r_V N_o) \quad (8272)$$

$$\tau^1_{\gamma,\alpha,w} = \sum_{a \in V} {}^2D^1_{a,w} W^1_{a,\alpha} Y^{1,*}_{a,\gamma} \quad (3r_D r_T r_V N_v) \quad (8273)$$

$$\tau^2_{\gamma,\alpha,w} = \sum_{i \in O} {}^2D^2_{i,w} W^2_{i,\alpha} Y^{2,*}_{i,\gamma} \quad (3r_D r_T r_V N_o) \quad (8274)$$

$$\tau^3_{\gamma,\alpha,w} = \sum_{\beta \in B} X_{\beta,\alpha} \tau^1_{\gamma,\beta,w} \tau^2_{\gamma,\beta,w} \quad (3r_D r_T r_V^2) \quad (8275)$$

$$\tau^4_{\gamma,\alpha,w} = \sum_{\delta \in A} Z^*_{\delta,\gamma} \tau^3_{\delta,\alpha,w} \quad (2r_D r_T^2 r_V) \quad (8276)$$

$$\tau^5_{\gamma,w,a} = \sum_{\alpha \in B} W^3_{a,\alpha} \tau^0_{\gamma,\alpha,w} \tau^4_{\gamma,\alpha,w} \quad (3r_D r_T r_V N_v) \quad (8277)$$

$${}^2R^3_{a,\gamma} \leftarrow \sum_{w \in D} {}^2D^3_{a,w} \tau^5_{\gamma,w,a} \quad (2r_D r_T N_v) \quad (8278)$$

## B. Contributions from $(H^1 T)_c$

Raw expression

$${}^2R^3_{b,\zeta} \leftarrow \sum_{\gamma \in A} \sum_{i \in O} \sum_{j \in O} \sum_{a \in V} \sum_{c \in V} {}^1T_{c,i} Y^{1,*}_{a,\gamma} Y^{2,*}_{i,\gamma} Z^*_{\gamma,\zeta} Y^{4,*}_{j,\zeta} {}^2D^{a,i,b,j}_{a,c,b,j} V_{a,c,b,j} \quad (8279)$$

Factorized expression

$$\tau^0_{\alpha,i} = \sum_{a \in V} {}^1T_{a,i} W^2_{a,\alpha} \quad (2r_V N_o N_v) \quad (8280)$$

$$\tau^1_{\gamma,\alpha,w} = \sum_{i \in O} {}^2D^2_{i,w} Y^{2,*}_{i,\gamma} \tau^0_{\alpha,i} \quad (3r_D r_T r_V N_o) \quad (8281)$$

$$\tau^2_{\gamma,\alpha,w} = \sum_{a \in V} {}^2D^1_{a,w} W^1_{a,\alpha} Y^{1,*}_{a,\gamma} \quad (3r_D r_T r_V N_v) \quad (8282)$$

$$\tau^3_{\gamma,\alpha,w} = \sum_{\beta \in B} X_{\beta,\alpha} \tau^1_{\gamma,\beta,w} \tau^2_{\gamma,\beta,w} \quad (3r_D r_T r_V^2) \quad (8283)$$

$$\tau^4_{\gamma,\alpha,w} = \sum_{\delta \in A} Z^*_{\delta,\gamma} \tau^3_{\delta,\alpha,w} \quad (2r_D r_T^2 r_V) \quad (8284)$$

$$\tau^5_{\gamma,\alpha,w} = \sum_{i \in O} {}^2D^4_{i,w} W^4_{i,\alpha} Y^{4,*}_{i,\gamma} \quad (3r_D r_T r_V N_o) \quad (8285)$$

$$\tau^6_{\gamma,w,a} = \sum_{\alpha \in B} W^3_{a,\alpha} \tau^4_{\gamma,\alpha,w} \tau^5_{\gamma,\alpha,w} \quad (3r_D r_T r_V N_v) \quad (8286)$$

$${}^2R^3_{a,\gamma} \leftarrow \sum_{w \in D} {}^2D^3_{a,w} \tau^6_{\gamma,w,a} \quad (2r_D r_T N_v) \quad (8287)$$

Raw expression

$${}^2R^3_{b,\zeta} \leftarrow \sum_{\gamma \in A} \sum_{i \in O} \sum_{j \in O} \sum_{a \in V} \sum_{c \in V} {}^1T_{c,j} Y^{1,*}_{a,\gamma} Y^{2,*}_{i,\gamma} Z^*_{\gamma,\zeta} Y^{4,*}_{j,\zeta} {}^2D^{a,i,b,j}_{a,i,b,c} V_{a,i,b,c} \quad (8288)$$

Factorized expression

$$\tau^0_{\gamma,\alpha,w} = \sum_{a \in V} {}^2D^1_{a,w} W^1_{a,\alpha} Y^{1,*}_{a,\gamma} \quad (3r_D r_T r_V N_v) \quad (8289)$$

$$\tau^1_{\gamma,\alpha,w} = \sum_{i \in O} {}^2D^2_{i,w} W^2_{i,\alpha} Y^{2,*}_{i,\gamma} \quad (3r_D r_T r_V N_o) \quad (8290)$$

$$\tau^2_{\gamma,\alpha,w} = \sum_{\beta \in B} X_{\beta,\alpha} \tau^0_{\gamma,\beta,w} \tau^1_{\gamma,\beta,w} \quad (3r_D r_T r_V^2) \quad (8291)$$

$$\tau^3_{\gamma,\alpha,w} = \sum_{\delta \in A} Z^*_{\delta,\gamma} \tau^2_{\delta,\alpha,w} \quad (2r_D r_T^2 r_V) \quad (8292)$$

$$\tau^4_{\alpha,i} = \sum_{a \in V} {}^1T_{a,i} W^4_{a,\alpha} \quad (2r_V N_o N_v) \quad (8293)$$

$$\tau^5_{\gamma,\alpha,w} = \sum_{i \in O} {}^2D^4_{i,w} Y^{4,*}_{i,\gamma} \tau^4_{\alpha,i} \quad (3r_D r_T r_V N_o) \quad (8294)$$

$$\tau^6_{\gamma,w,a} = \sum_{\alpha \in B} W^3_{a,\alpha} \tau^3_{\gamma,\alpha,w} \tau^5_{\gamma,\alpha,w} \quad (3r_D r_T r_V N_v) \quad (8295)$$

$${}^2R^3_{a,\gamma} \leftarrow \sum_{w \in D} {}^2D^3_{a,w} \tau^6_{\gamma,w,a} \quad (2r_D r_T N_v) \quad (8296)$$

Raw expression

$${}^2R^3_{b,\zeta} \leftarrow - \sum_{\gamma \in A} \sum_{i \in O} \sum_{j \in O} \sum_{k \in O} \sum_{a \in V} {}^1T_{a,k} Y^{1,*}_{a,\gamma} Y^{2,*}_{i,\gamma} Z^*_{\gamma,\zeta} Y^{4,*}_{j,\zeta} {}^2D^{a,i,b,j}_{V_{b,j,k,i}} \quad (8297)$$

Factorized expression

$$\tau^0_{\gamma,\alpha,w} = \sum_{i \in O} {}^2D^4_{i,w} W^2_{i,\alpha} Y^{4,*}_{i,\gamma} \quad (3r_D r_T r_V N_o) \quad (8298)$$

$$\tau^1_{\gamma,w,i} = \sum_{a \in V} {}^2D^1_{a,w} {}^1T_{a,i} Y^{1,*}_{a,\gamma} \quad (3r_D r_T N_o N_v) \quad (8299)$$

$$\tau^2_{\gamma,\alpha,w} = \sum_{i \in O} W^3_{i,\alpha} \tau^1_{\gamma,w,i} \quad (2r_D r_T r_V N_o) \quad (8300)$$

$$\tau^3_{\gamma,\alpha,w} = \sum_{i \in O} {}^2D^2_{i,w} W^4_{i,\alpha} Y^{2,*}_{i,\gamma} \quad (3r_D r_T r_V N_o) \quad (8301)$$

$$\tau^4_{\gamma,\alpha,w} = \sum_{\beta \in B} X_{\alpha,\beta} \tau^2_{\gamma,\beta,w} \tau^3_{\gamma,\beta,w} \quad (3r_D r_T r_V^2) \quad (8302)$$

$$\tau^5_{\gamma,\alpha,w} = \sum_{\delta \in A} Z^*_{\delta,\gamma} \tau^4_{\delta,\alpha,w} \quad (2r_D r_T^2 r_V) \quad (8303)$$

$$\tau^6_{\gamma,w,a} = \sum_{\alpha \in B} W^1_{a,\alpha} \tau^0_{\gamma,\alpha,w} \tau^5_{\gamma,\alpha,w} \quad (3r_D r_T r_V N_v) \quad (8304)$$

$${}^2R^3_{a,\gamma} \leftarrow - \sum_{w \in D} {}^2D^3_{a,w} \tau^6_{\gamma,w,a} \quad (2r_D r_T N_v) \quad (8305)$$

Raw expression

$${}^2R^3_{b,\zeta} \leftarrow - \sum_{\gamma \in A} \sum_{i \in O} \sum_{j \in O} \sum_{k \in O} \sum_{a \in V} {}^1T_{b,k} Y^{1,*}_{a,\gamma} Y^{2,*}_{i,\gamma} Z^*_{\gamma,\zeta} Y^{4,*}_{j,\zeta} {}^2D^{a,i,b,j}_{V_{a,i,k,j}} \quad (8306)$$

Factorized expression

$$\tau^0_{\gamma,\alpha,w} = \sum_{i \in O} {}^2D^4_{i,w} W^4_{i,\alpha} Y^{4,*}_{i,\gamma} \quad (3r_D r_T r_V N_o) \quad (8307)$$

$$\tau^1_{\gamma,\alpha,w} = \sum_{a \in V} {}^2D^1_{a,w} W^1_{a,\alpha} Y^{1,*}_{a,\gamma} \quad (3r_D r_T r_V N_v) \quad (8308)$$

$$\tau^2_{\gamma,\alpha,w} = \sum_{i \in O} {}^2D^2_{i,w} W^2_{i,\alpha} Y^{2,*}_{i,\gamma} \quad (3r_D r_T r_V N_o) \quad (8309)$$

$$\tau^3_{\gamma,\alpha,w} = \sum_{\beta \in B} X_{\beta,\alpha} \tau^1_{\gamma,\beta,w} \tau^2_{\gamma,\beta,w} \quad (3r_D r_T r_V^2) \quad (8310)$$

$$\tau^4_{\gamma,\alpha,w} = \sum_{\delta \in A} Z^*_{\delta,\gamma} \tau^3_{\delta,\alpha,w} \quad (2r_D r_T^2 r_V) \quad (8311)$$

$$\tau^5_{\gamma,w,i} = \sum_{\alpha \in B} W^3_{i,\alpha} \tau^0_{\gamma,\alpha,w} \tau^4_{\gamma,\alpha,w} \quad (3r_D r_T r_V N_o) \quad (8312)$$

$${}^2R^3_{a,\gamma} \leftarrow - \sum_{w \in D} \sum_{i \in O} {}^2D^3_{a,w} {}^1T_{a,i} \tau^5_{\gamma,w,i} \quad (3r_D r_T N_o N_v) \quad (8313)$$

### C. Contributions from $(H^1 T^1 T)_c$

Raw expression

$${}^2R^3_{b,\zeta} \leftarrow \sum_{\gamma \in A} \sum_{i \in O} \sum_{j \in O} \sum_{a \in V} \sum_{c \in V} \sum_{d \in V} {}^1T_{c,i} {}^1T_{d,j} Y^{1,*}_{a,\gamma} Y^{2,*}_{i,\gamma} Z^*_{\gamma,\zeta} Y^{4,*}_{j,\zeta} {}^2D^{a,i,b,j}_{V_{a,c,b,d}} \quad (8314)$$

Factorized expression

$$\tau^0_{\gamma,w,i} = \sum_{a \in V} {}^2D^1_{a,w} {}^1T_{a,i} Y^{1,*}_{a,\gamma} \quad (3r_D r_T N_o N_v) \quad (8315)$$

$$\tau^1_{\gamma,\alpha,w} = \sum_{i \in O} W^1_{i,\alpha} \tau^0_{\gamma,w,i} \quad (2r_D r_T r_V N_o) \quad (8316)$$

$$\tau^2_{\gamma,\alpha,w} = \sum_{i \in O} {}^2D^2_{i,w} W^2_{i,\alpha} Y^{2,*}_{i,\gamma} \quad (3r_D r_T r_V N_o) \quad (8317)$$

$$\tau^3_{\gamma,\alpha,w} = \sum_{\beta \in B} X_{\beta,\alpha} \tau^1_{\gamma,\beta,w} \tau^2_{\gamma,\beta,w} \quad (3r_D r_T r_V^2) \quad (8318)$$

$$\tau^4_{\gamma,\alpha,w} = \sum_{\delta \in A} Z^*_{\delta,\gamma} \tau^3_{\delta,\alpha,w} \quad (2r_D r_T^2 r_V) \quad (8319)$$

$$\tau^5_{\gamma,\alpha,w} = \sum_{i \in O} {}^2D^4_{i,w} W^4_{i,\alpha} Y^{4,*}_{i,\gamma} \quad (3r_D r_T r_V N_o) \quad (8320)$$

$$\tau^6_{\gamma,w,i} = \sum_{\alpha \in B} W^3_{i,\alpha} \tau^4_{\gamma,\alpha,w} \tau^5_{\gamma,\alpha,w} \quad (3r_D r_T r_V N_o) \quad (8321)$$

$${}^2R^3_{a,\gamma} \leftarrow \sum_{w \in D} \sum_{i \in O} {}^2D^3_{a,w} {}^1T_{a,i} \tau^6_{\gamma,w,i} \quad (3r_D r_T N_o N_v) \quad (8322)$$

Raw expression

$${}^2R^3_{b,\zeta} \leftarrow - \sum_{\gamma \in A} \sum_{i \in O} \sum_{j \in O} \sum_{k \in O} \sum_{a \in V} \sum_{c \in V} {}^1T_{a,k} {}^1T_{c,i} Y^{1,*}_{a,\gamma} Y^{2,*}_{i,\gamma} Z^*_{\gamma,\zeta} Y^{4,*}_{j,\zeta} {}^2D^{a,i,b,j}_{V_{b,j,k,c}} \quad (8323)$$

Factorized expression

$$\tau^0_{\alpha,i} = \sum_{a \in V} {}^1T_{a,i} W^4_{a,\alpha} \quad (2r_V N_o N_v) \quad (8324)$$

$$\tau^1_{\gamma,\alpha,w} = \sum_{i \in O} {}^2D^4_{i,w} Y^{4,*}_{i,\gamma} \tau^0_{\alpha,i} \quad (3r_D r_T r_V N_o) \quad (8325)$$

$$\tau^2_{\alpha,i} = \sum_{a \in V} {}^1T_{a,i} W^2_{a,\alpha} \quad (2r_V N_o N_v) \quad (8326)$$

$$\tau^3_{\gamma,\alpha,w} = \sum_{i \in O} {}^2D^2_{i,w} Y^{2,*}_{i,\gamma} \tau^2_{\alpha,i} \quad (3r_D r_T r_V N_o) \quad (8327)$$

$$\tau^4_{\gamma,\alpha,w} = \sum_{a \in V} {}^2D^1_{a,w} W^1_{a,\alpha} Y^{1,*}_{a,\gamma} \quad (3r_D r_T r_V N_v) \quad (8328)$$

$$\tau^5_{\gamma,\alpha,w} = \sum_{\beta \in B} X_{\beta,\alpha} \tau^3_{\gamma,\beta,w} \tau^4_{\gamma,\beta,w} \quad (3r_D r_T r_V^2) \quad (8329)$$

$$\tau^6_{\gamma,\alpha,w} = \sum_{\delta \in A} Z^*_{\delta,\gamma} \tau^5_{\delta,\alpha,w} \quad (2r_D r_T^2 r_V) \quad (8330)$$

$$\tau^7_{\gamma,w,a} = \sum_{\alpha \in B} W^3_{a,\alpha} \tau^1_{\gamma,\alpha,w} \tau^6_{\gamma,\alpha,w} \quad (3r_D r_T r_V N_v) \quad (8331)$$

$${}^2R^3_{a,\gamma} \leftarrow \sum_{w \in D} {}^2D^3_{a,w} \tau^7_{\gamma,w,a} \quad (2r_D r_T N_v) \quad (8332)$$

Raw expression

$${}^2R^3_{b,\zeta} \leftarrow - \sum_{\gamma \in A} \sum_{i \in O} \sum_{j \in O} \sum_{k \in O} \sum_{a \in V} \sum_{c \in V} {}^1T_{a,k} {}^1T_{c,j} Y^{1,*}_{a,\gamma} Y^{2,*}_{i,\gamma} Z^*_{\gamma,\zeta} Y^{4,*}_{j,\zeta} {}^2D^{a,i,b,j}_{V_{b,c,k,i}} \quad (8333)$$

Factorized expression

$$\tau^0_{\gamma,\alpha,w} = \sum_{i \in O} {}^2D^4_{i,w} W^2_{i,\alpha} Y^{4,*}_{i,\gamma} \quad (3r_D r_T r_V N_o) \quad (8334)$$

$$\tau^1_{\alpha,i} = \sum_{a \in V} {}^1T_{a,i} W^4_{a,\alpha} \quad (2r_V N_o N_v) \quad (8335)$$

$$\tau^2_{\gamma,\alpha,w} = \sum_{i \in O} {}^2D^2_{i,w} Y^{2,*}_{i,\gamma} \tau^1_{\alpha,i} \quad (3r_D r_T r_V N_o) \quad (8336)$$

$$\tau^3_{\gamma,w,i} = \sum_{a \in V} {}^2D^1_{a,w} {}^1T_{a,i} Y^{1,*}_{a,\gamma} \quad (3r_D r_T N_o N_v) \quad (8337)$$

$$\tau^4_{\gamma,\alpha,w} = \sum_{i \in O} W^3_{i,\alpha} \tau^3_{\gamma,w,i} \quad (2r_D r_T r_V N_o) \quad (8338)$$

$$\tau^5_{\gamma,\alpha,w} = \sum_{\beta \in B} X_{\alpha,\beta} \tau^2_{\gamma,\beta,w} \tau^4_{\gamma,\beta,w} \quad (3r_D r_T r_V^2) \quad (8339)$$

$$\tau^6_{\gamma,\alpha,w} = \sum_{\delta \in A} Z^*_{\delta,\gamma} \tau^5_{\delta,\alpha,w} \quad (2r_D r_T^2 r_V) \quad (8340)$$

$$\tau^7_{\gamma,w,a} = \sum_{\alpha \in B} W^1_{a,\alpha} \tau^0_{\gamma,\alpha,w} \tau^6_{\gamma,\alpha,w} \quad (3r_D r_T r_V N_v) \quad (8341)$$

$${}^2R^3_{a,\gamma} \leftarrow - \sum_{w \in D} {}^2D^3_{a,w} \tau^7_{\gamma,w,a} \quad (2r_D r_T N_v) \quad (8342)$$

Raw expression

$${}^2R^3_{b,\zeta} \leftarrow - \sum_{\gamma \in A} \sum_{i \in O} \sum_{j \in O} \sum_{k \in O} \sum_{a \in V} \sum_{c \in V} {}^1T_{b,k} {}^1T_{c,i} Y^{1,*}_{a,\gamma} Y^{2,*}_{i,\gamma} Z^*_{\gamma,\zeta} Y^{4,*}_{j,\zeta} {}^2D^{a,i,b,j}_{V_{a,c,k,j}} \quad (8343)$$

Factorized expression

$$\tau^0_{\gamma,w,i} = \sum_{a \in V} {}^2D^1_{a,w} {}^1T_{a,i} Y^{1,*}_{a,\gamma} \quad (3r_D r_T N_o N_v) \quad (8344)$$

$$\tau^1_{\gamma,\alpha,w} = \sum_{i \in O} W^3_{i,\alpha} \tau^0_{\gamma,w,i} \quad (2r_D r_T r_V N_o) \quad (8345)$$

$$\tau^2_{\gamma,\alpha,w} = \sum_{i \in O} {}^2D^2_{i,w} W^4_{i,\alpha} Y^{2,*}_{i,\gamma} \quad (3r_D r_T r_V N_o) \quad (8346)$$

$$\tau^3_{\gamma,\alpha,w} = \sum_{\beta \in B} X_{\alpha,\beta} \tau^1_{\gamma,\beta,w} \tau^2_{\gamma,\beta,w} \quad (3r_D r_T r_V^2) \quad (8347)$$

$$\tau^4_{\gamma,\alpha,w} = \sum_{\delta \in A} Z^*_{\delta,\gamma} \tau^3_{\delta,\alpha,w} \quad (2r_D r_T^2 r_V) \quad (8348)$$

$$\tau^5_{\alpha,i} = \sum_{a \in V} {}^1T_{a,i} W^2_{a,\alpha} \quad (2r_V N_o N_v) \quad (8349)$$

$$\tau^6_{\gamma,\alpha,w} = \sum_{i \in O} {}^2D^4_{i,w} Y^{4,*}_{i,\gamma} \tau^5_{\alpha,i} \quad (3r_D r_T r_V N_o) \quad (8350)$$

$$\tau^7_{\gamma,w,a} = \sum_{\alpha \in B} W^1_{a,\alpha} \tau^4_{\gamma,\alpha,w} \tau^6_{\gamma,\alpha,w} \quad (3r_D r_T r_V N_v) \quad (8351)$$

$${}^2R^3_{a,\gamma} \leftarrow - \sum_{w \in D} {}^2D^3_{a,w} \tau^7_{\gamma,w,a} \quad (2r_D r_T N_v) \quad (8352)$$

Raw expression

$${}^2R^3_{b,\zeta} \leftarrow - \sum_{\gamma \in A} \sum_{i \in O} \sum_{j \in O} \sum_{k \in O} \sum_{a \in V} \sum_{c \in V} {}^1T_{b,k} {}^1T_{c,j} Y^{1,*}_{a,\gamma} Y^{2,*}_{i,\gamma} Z^*_{\gamma,\zeta} Y^{4,*}_{j,\zeta} {}^2D^{a,i,b,j}_{V_{a,i,k,c}} \quad (8353)$$

Factorized expression

$$\tau^0_{\alpha,i} = \sum_{a \in V} {}^1T_{a,i} W^2_{a,\alpha} \quad (2r_V N_o N_v) \quad (8354)$$

$$\tau^1_{\gamma,\alpha,w} = \sum_{i \in O} {}^2D^2_{i,w} Y^{2,*}_{i,\gamma} \tau^0_{\alpha,i} \quad (3r_D r_T r_V N_o) \quad (8355)$$

$$\tau^2_{\gamma,\alpha,w} = \sum_{a \in V} {}^2D^1_{a,w} W^1_{a,\alpha} Y^{1,*}_{a,\gamma} \quad (3r_D r_T r_V N_v) \quad (8356)$$

$$\tau^3_{\gamma,\alpha,w} = \sum_{\beta \in B} X_{\beta,\alpha} \tau^1_{\gamma,\beta,w} \tau^2_{\gamma,\beta,w} \quad (3r_D r_T r_V^2) \quad (8357)$$

$$\tau^4_{\gamma,\alpha,w} = \sum_{\delta \in A} Z^*_{\delta,\gamma} \tau^3_{\delta,\alpha,w} \quad (2r_D r_T^2 r_V) \quad (8358)$$

$$\tau^5_{\gamma,\alpha,w} = \sum_{i \in O} {}^2D^4_{i,w} W^4_{i,\alpha} Y^{4,*}_{i,\gamma} \quad (3r_D r_T r_V N_o) \quad (8359)$$

$$\tau^6_{\gamma,w,i} = \sum_{\alpha \in B} W^3_{i,\alpha} \tau^4_{\gamma,\alpha,w} \tau^5_{\gamma,\alpha,w} \quad (3r_D r_T r_V N_o) \quad (8360)$$

$${}^2R^3_{a,\gamma} \leftarrow - \sum_{w \in D} \sum_{i \in O} {}^2D^3_{a,w} {}^1T_{a,i} \tau^6_{\gamma,w,i} \quad (3r_D r_T N_o N_v) \quad (8361)$$

Raw expression

$${}^2R^3_{b,\zeta} \leftarrow \sum_{\gamma \in A} \sum_{i \in O} \sum_{j \in O} \sum_{k \in O} \sum_{l \in O} \sum_{a \in V} {}^1T_{a,l} {}^1T_{b,k} Y^{1,*}_{a,\gamma} Y^{2,*}_{i,\gamma} Z^*_{\gamma,\zeta} Y^{4,*}_{j,\zeta} {}^2D^{a,i,b,j}_{V_{l,i,k,j}} \quad (8362)$$

Factorized expression

$$\tau^0_{\gamma,\alpha,w} = \sum_{a \in V} {}^2D^1_{a,w} W^1_{a,\alpha} Y^{1,*}_{a,\gamma} \quad (3r_D r_T r_V N_v) \quad (8363)$$

$$\tau^1_{\gamma,\alpha,w} = \sum_{i \in O} {}^2D^2_{i,w} W^2_{i,\alpha} Y^{2,*}_{i,\gamma} \quad (3r_D r_T r_V N_o) \quad (8364)$$

$$\tau^2_{\gamma,\alpha,w} = \sum_{\beta \in B} X_{\beta,\alpha} \tau^0_{\gamma,\beta,w} \tau^1_{\gamma,\beta,w} \quad (3r_D r_T r_V^2) \quad (8365)$$

$$\tau^3_{\gamma,\alpha,w} = \sum_{\delta \in A} Z^*_{\delta,\gamma} \tau^2_{\delta,\alpha,w} \quad (2r_D r_T^2 r_V) \quad (8366)$$



$$\tau_{\alpha,i}^4 = \sum_{a \in V} {}^1T_{a,i} W_{a,\alpha}^4 \quad (2r_V N_o N_v) \quad (8367)$$

$$\tau_{\gamma,\alpha,w}^5 = \sum_{i \in O} {}^2D_{i,w}^4 Y_{i,\gamma}^{4,*} \tau_{\alpha,i}^4 \quad (3r_D r_T r_V N_o) \quad (8368)$$

$$\tau_{\gamma,w,i}^6 = \sum_{\alpha \in B} W_{i,\alpha}^3 \tau_{\gamma,\alpha,w}^3 \tau_{\gamma,\alpha,w}^5 \quad (3r_D r_T r_V N_o) \quad (8369)$$

$${}^2R_{a,\gamma}^3 \leftarrow - \sum_{w \in D} \sum_{i \in O} {}^2D_{a,w}^3 {}^1T_{a,i} \tau_{\gamma,w,i}^6 \quad (3r_D r_T N_o N_v) \quad (8370)$$

#### D. Contributions from $(H^2T)_c$

Raw expression

$${}^2R_{b,\zeta}^3 \leftarrow \sum_{\gamma \in A} \sum_{i \in O} \sum_{j \in O} \sum_{a \in V} \sum_{c \in V} \sum_{d \in V} \frac{1}{2} Y_{a,\gamma}^{1,*} Y_{i,\gamma}^{2,*} Z_{\gamma,\zeta}^* Y_{j,\zeta}^{4,*} {}^2D_{a,i,b,j} {}^2T_{c,i,d,j} V_{a,c,b,d} \quad (8371)$$

Factorized expression

$$\tau_{\gamma,\alpha,w}^0 = \sum_{i \in O} {}^2D_{i,w}^2 W_{i,\alpha}^2 Y_{i,\gamma}^{2,*} \quad (3r_D r_T r_V N_o) \quad (8372)$$

$$\tau_{\gamma,\delta,w}^1 = \sum_{a \in V} {}^2D_{a,w}^1 Y_{a,\gamma}^1 Y_{a,\delta}^{1,*} \quad (3r_D r_T^2 N_v) \quad (8373)$$

$$\tau_{\gamma,\delta,w,i}^2 = \sum_{\epsilon \in A} Y_{i,\epsilon}^2 Z_{\epsilon,\gamma} \tau_{\epsilon,\delta,w}^1 \quad (3r_D r_T^3 N_o) \quad (8374)$$

$$\tau_{\gamma,\delta,\alpha,w}^3 = \sum_{i \in O} W_{i,\alpha}^1 \tau_{\delta,\alpha,w}^0 \tau_{\gamma,\delta,w,i}^2 \quad (3r_D r_T^2 r_V N_o) \quad (8375)$$

$$\tau_{\alpha,i,j}^4 = \sum_{\beta \in B} X_{\alpha,\beta} W_{i,\beta}^3 W_{j,\beta}^4 \quad (3r_V^2 N_o^2) \quad (8376)$$

$$\tau_{\gamma,\alpha,i}^5 = \sum_{j \in O} Y_{j,\gamma}^4 \tau_{\alpha,j,i}^4 \quad (2r_T r_V N_o^2) \quad (8377)$$

$$\tau_{\gamma,\delta,w,i}^6 = \sum_{\alpha \in B} \tau_{\gamma,\alpha,i}^5 \tau_{\gamma,\delta,\alpha,w}^3 \quad (2r_D r_T^2 r_V N_o) \quad (8378)$$

$$\tau_{\gamma,\delta,w}^7 = \sum_{\epsilon \in A} \sum_{i \in O} {}^2D_{i,w}^4 Z_{\epsilon,\delta}^* Y_{i,\delta}^{4,*} \tau_{\gamma,\epsilon,w,i}^6 \quad (4r_D r_T^3 N_o) \quad (8379)$$

$${}^2R_{a,\gamma}^3 \leftarrow \sum_{\delta \in A} \sum_{w \in D} \frac{1}{2} {}^2D_{a,w}^3 Y_{a,\delta}^3 \tau_{\delta,\gamma,w}^7 \quad (3r_D r_T^2 N_v) \quad (8380)$$

Raw expression

$${}^2R_{b,\zeta}^3 \leftarrow \sum_{\gamma \in A} \sum_{i \in O} \sum_{j \in O} \sum_{a \in V} \sum_{c \in V} \sum_{d \in V} \frac{1}{2} Y_{a,\gamma}^{1,*} Y_{i,\gamma}^{2,*} Z_{\gamma,\zeta}^* Y_{j,\zeta}^{4,*} {}^2D_{a,i,b,j} {}^2T_{c,j,d,i} V_{a,d,b,c} \quad (8381)$$

Factorized expression

$$\tau_{\gamma,\alpha,w}^0 = \sum_{i \in O} {}^2D_{i,w}^2 W_{i,\alpha}^2 Y_{i,\gamma}^{2,*} \quad (3r_D r_T r_V N_o) \quad (8382)$$

$$\tau_{\gamma,\delta,w}^1 = \sum_{a \in V} {}^2D_{a,w}^1 Y_{a,\gamma}^3 Y_{a,\delta}^{1,*} \quad (3r_D r_T^2 N_v) \quad (8383)$$

$$\tau_{\gamma,\delta,w,i}^2 = \sum_{\epsilon \in A} Z_{\gamma,\epsilon} Y_{i,\epsilon}^4 \tau_{\epsilon,\delta,w}^1 \quad (3r_D r_T^3 N_o) \quad (8384)$$

$$\tau_{\gamma,\delta,\alpha,w}^3 = \sum_{i \in O} W_{i,\alpha}^1 \tau_{\delta,\alpha,w}^0 \tau_{\gamma,\delta,w,i}^2 \quad (3r_D r_T^2 r_V N_o) \quad (8385)$$

$$\tau_{\alpha,i,j}^4 = \sum_{\beta \in B} X_{\alpha,\beta} W_{i,\beta}^3 W_{j,\beta}^4 \quad (3r_V^2 N_o^2) \quad (8386)$$

$$\tau_{\gamma,\alpha,i}^5 = \sum_{j \in O} Y_{j,\gamma}^2 \tau_{\alpha,j,i}^4 \quad (2r_T r_V N_o^2) \quad (8387)$$

$$\tau_{\gamma,\delta,w,i}^6 = \sum_{\alpha \in B} \tau_{\gamma,\alpha,i}^5 \tau_{\gamma,\delta,\alpha,w}^3 \quad (2r_D r_T^2 r_V N_o) \quad (8388)$$

$$\tau_{\gamma,\delta,w}^7 = \sum_{\epsilon \in A} \sum_{i \in O} {}^2D_{i,w}^4 Z_{\epsilon,\delta}^* Y_{i,\delta}^{4,*} \tau_{\gamma,\epsilon,w,i}^6 \quad (4r_D r_T^3 N_o) \quad (8389)$$

$${}^2R_{a,\gamma}^3 \leftarrow \sum_{\delta \in A} \sum_{w \in D} \frac{1}{2} {}^2D_{a,w}^3 Y_{a,\delta}^1 \tau_{\delta,\gamma,w}^7 \quad (3r_D r_T^2 N_v) \quad (8390)$$

Raw expression

$${}^2R^3_{b,\zeta} \leftarrow \sum_{\gamma \in A} \sum_{i \in O} \sum_{j \in O} \sum_{k \in O} \sum_{a \in V} \sum_{c \in V} Y^{1,*}_{a,\gamma} Y^{2,*}_{i,\gamma} Z^*_{\gamma,\zeta} Y^{4,*}_{j,\zeta} {}^2D^{a,i,b,j} {}^2T_{a,i,c,k} V_{b,j,k,c} \quad (8391)$$

Factorized expression

$$\tau^0_{\gamma,\delta,w} = \sum_{i \in O} {}^2D^4_{i,w} Y^2_{i,\gamma} Y^{4,*}_{i,\delta} \quad (3r_D r_T^2 N_o) \quad (8392)$$

$$\tau^1_{\gamma,\alpha,w} = \sum_{a \in V} {}^2D^1_{a,w} W^1_{a,\alpha} Y^{1,*}_{a,\gamma} \quad (3r_D r_T r_V N_v) \quad (8393)$$

$$\tau^2_{\gamma,\alpha,w} = \sum_{i \in O} {}^2D^2_{i,w} W^2_{i,\alpha} Y^{2,*}_{i,\gamma} \quad (3r_D r_T r_V N_o) \quad (8394)$$

$$\tau^3_{\gamma,\alpha} = \sum_{a \in V} W^4_{a,\alpha} Y^3_{a,\gamma} \quad (2r_T r_V N_v) \quad (8395)$$

$$\tau^4_{\gamma,\alpha} = \sum_{i \in O} W^3_{i,\alpha} Y^4_{i,\gamma} \quad (2r_T r_V N_o) \quad (8396)$$

$$\tau^5_{\gamma,\alpha} = \sum_{\beta \in B} X_{\alpha,\beta} \tau^3_{\gamma,\beta} \tau^4_{\gamma,\beta} \quad (3r_T r_V^2) \quad (8397)$$

$$\tau^6_{\gamma,\alpha} = \sum_{\delta \in A} Z_{\gamma,\delta} \tau^5_{\delta,\alpha} \quad (2r_T^2 r_V) \quad (8398)$$

$$\tau^7_{\gamma,\delta,w} = \sum_{\alpha \in B} \tau^6_{\gamma,\alpha} \tau^1_{\delta,\alpha,w} \tau^2_{\delta,\alpha,w} \quad (3r_D r_T^2 r_V) \quad (8399)$$

$$\tau^8_{\gamma,\delta,w} = \sum_{\epsilon \in A} Z^*_{\epsilon,\delta} \tau^7_{\gamma,\epsilon,w} \quad (2r_D r_T^3) \quad (8400)$$

$${}^2R^3_{a,\gamma} \leftarrow \sum_{\delta \in A} \sum_{w \in D} {}^2D^3_{a,w} Y^1_{a,\delta} \tau^0_{\delta,\gamma,w} \tau^8_{\delta,\gamma,w} \quad (4r_D r_T^2 N_v) \quad (8401)$$

Raw expression

$${}^2R^3_{b,\zeta} \leftarrow \sum_{\gamma \in A} \sum_{i \in O} \sum_{j \in O} \sum_{k \in O} \sum_{a \in V} \sum_{c \in V} Y^{1,*}_{a,\gamma} Y^{2,*}_{i,\gamma} Z^*_{\gamma,\zeta} Y^{4,*}_{j,\zeta} {}^2D^{a,i,b,j} {}^2T_{b,j,c,k} V_{a,i,k,c} \quad (8402)$$

Factorized expression

$$\tau^0_{\gamma,\delta,w} = \sum_{i \in O} {}^2D^4_{i,w} Y^4_{i,\gamma} Y^{4,*}_{i,\delta} \quad (3r_D r_T^2 N_o) \quad (8403)$$

$$\tau^1_{\gamma,\alpha,w} = \sum_{a \in V} {}^2D^1_{a,w} W^1_{a,\alpha} Y^{1,*}_{a,\gamma} \quad (3r_D r_T r_V N_v) \quad (8404)$$

$$\tau^2_{\gamma,\alpha,w} = \sum_{i \in O} {}^2D^2_{i,w} W^2_{i,\alpha} Y^{2,*}_{i,\gamma} \quad (3r_D r_T r_V N_o) \quad (8405)$$

$$\tau^3_{\gamma,\alpha} = \sum_{a \in V} W^4_{a,\alpha} Y^1_{a,\gamma} \quad (2r_T r_V N_v) \quad (8406)$$

$$\tau^4_{\gamma,\alpha} = \sum_{i \in O} W^3_{i,\alpha} Y^2_{i,\gamma} \quad (2r_T r_V N_o) \quad (8407)$$

$$\tau^5_{\gamma,\alpha} = \sum_{\beta \in B} X_{\alpha,\beta} \tau^3_{\gamma,\beta} \tau^4_{\gamma,\beta} \quad (3r_T r_V^2) \quad (8408)$$

$$\tau^6_{\gamma,\alpha} = \sum_{\delta \in A} Z_{\delta,\gamma} \tau^5_{\delta,\alpha} \quad (2r_T^2 r_V) \quad (8409)$$

$$\tau^7_{\gamma,\delta,w} = \sum_{\alpha \in B} \tau^6_{\gamma,\alpha} \tau^1_{\delta,\alpha,w} \tau^2_{\delta,\alpha,w} \quad (3r_D r_T^2 r_V) \quad (8410)$$

$$\tau^8_{\gamma,\delta,w} = \sum_{\epsilon \in A} Z^*_{\epsilon,\delta} \tau^7_{\gamma,\epsilon,w} \quad (2r_D r_T^3) \quad (8411)$$

$${}^2R^3_{a,\gamma} \leftarrow \sum_{\delta \in A} \sum_{w \in D} {}^2D^3_{a,w} Y^3_{a,\delta} \tau^0_{\delta,\gamma,w} \tau^8_{\delta,\gamma,w} \quad (4r_D r_T^2 N_v) \quad (8412)$$

Raw expression

$${}^2R^3_{b,\zeta} \leftarrow \sum_{\gamma \in A} \sum_{i \in O} \sum_{j \in O} \sum_{k \in O} \sum_{a \in V} \sum_{c \in V} Y^{1,*}_{a,\gamma} Y^{2,*}_{i,\gamma} Z^*_{\gamma,\zeta} Y^{4,*}_{j,\zeta} {}^2D^{a,i,b,j} {}^2T_{c,k,a,i} V_{b,j,k,c} \quad (8413)$$

Factorized expression

$$\tau^0_{\gamma,\alpha,w} = \sum_{i \in O} {}^2D^4_{i,w} W^2_{i,\alpha} Y^{4,*}_{i,\gamma} \quad (3r_D r_T r_V N_o) \quad (8414)$$

$$\tau^1_{\gamma,\alpha} = \sum_{a \in V} W^4_{a,\alpha} Y^3_{a,\gamma} \quad (2r_T r_V N_v) \quad (8415)$$

$$\tau^2_{\gamma,\alpha} = \sum_{i \in O} W^3_{i,\alpha} Y^4_{i,\gamma} \quad (2r_T r_V N_o) \quad (8416)$$

$$\tau^3_{\gamma,\alpha} = \sum_{\beta \in B} X_{\alpha,\beta} \tau^1_{\gamma,\beta} \tau^2_{\gamma,\beta} \quad (3r_T r_V^2) \quad (8417)$$

$$\tau^4_{\gamma,\alpha} = \sum_{\delta \in A} Z_{\gamma,\delta} \tau^3_{\delta,\alpha} \quad (2r_T^2 r_V) \quad (8418)$$

$$\tau^5_{\gamma,\delta,w} = \sum_{a \in V} {}^2D^1_{a,w} Y^1_{a,\gamma} Y^{1,*}_{a,\delta} \quad (3r_D r_T^2 N_v) \quad (8419)$$

$$\tau^6_{\gamma,\delta,w} = \sum_{i \in O} {}^2D^2_{i,w} Y^2_{i,\gamma} Y^{2,*}_{i,\delta} \quad (3r_D r_T^2 N_o) \quad (8420)$$

$$\tau^7_{\gamma,\delta,w} = \sum_{\epsilon \in A} Z^*_{\epsilon,\delta} \tau^5_{\gamma,\epsilon,w} \tau^6_{\gamma,\epsilon,w} \quad (3r_D r_T^3) \quad (8421)$$

$$\tau^8_{\gamma,\alpha,w} = \sum_{\delta \in A} \tau^4_{\delta,\alpha} \tau^7_{\delta,\gamma,w} \quad (2r_D r_T^2 r_V) \quad (8422)$$

$$\tau^9_{\gamma,w,a} = \sum_{\alpha \in B} W^1_{a,\alpha} \tau^0_{\gamma,\alpha,w} \tau^8_{\gamma,\alpha,w} \quad (3r_D r_T r_V N_v) \quad (8423)$$

$${}^2R^3_{a,\gamma} \leftarrow \sum_{w \in D} {}^2D^3_{a,w} \tau^9_{\gamma,w,a} \quad (2r_D r_T N_v) \quad (8424)$$

Raw expression

$${}^2R^3_{b,\zeta} \leftarrow \sum_{\gamma \in A} \sum_{i \in O} \sum_{j \in O} \sum_{k \in O} \sum_{a \in V} \sum_{c \in V} Y^{1,*}_{a,\gamma} Y^{2,*}_{i,\gamma} Z^*_{\gamma,\zeta} Y^{4,*}_{j,\zeta} {}^2D^{a,i,b,j} {}^2T_{c,k,b,j} V_{a,i,k,c} \quad (8425)$$

Factorized expression

$$\tau^0_{\gamma,\alpha,w} = \sum_{i \in O} {}^2D^4_{i,w} W^2_{i,\alpha} Y^{4,*}_{i,\gamma} \quad (3r_D r_T r_V N_o) \quad (8426)$$

$$\tau^1_{\gamma,\delta,w} = \sum_{a \in V} {}^2D^1_{a,w} Y^3_{a,\gamma} Y^{1,*}_{a,\delta} \quad (3r_D r_T^2 N_v) \quad (8427)$$

$$\tau^2_{\gamma,\delta,w} = \sum_{i \in O} {}^2D^2_{i,w} Y^4_{i,\gamma} Y^{2,*}_{i,\delta} \quad (3r_D r_T^2 N_o) \quad (8428)$$

$$\tau^3_{\gamma,\delta,w} = \sum_{\epsilon \in A} Z^*_{\epsilon,\delta} \tau^1_{\gamma,\epsilon,w} \tau^2_{\gamma,\epsilon,w} \quad (3r_D r_T^3) \quad (8429)$$

$$\tau^4_{\gamma,\alpha} = \sum_{a \in V} W^4_{a,\alpha} Y^1_{a,\gamma} \quad (2r_T r_V N_v) \quad (8430)$$

$$\tau^5_{\gamma,\alpha} = \sum_{i \in O} W^3_{i,\alpha} Y^2_{i,\gamma} \quad (2r_T r_V N_o) \quad (8431)$$

$$\tau^6_{\gamma,\alpha} = \sum_{\beta \in B} X_{\alpha,\beta} \tau^4_{\gamma,\beta} \tau^5_{\gamma,\beta} \quad (3r_T r_V^2) \quad (8432)$$

$$\tau^7_{\gamma,\alpha} = \sum_{\delta \in A} Z_{\delta,\gamma} \tau^6_{\delta,\alpha} \quad (2r_T^2 r_V) \quad (8433)$$

$$\tau^8_{\gamma,\alpha,w} = \sum_{\delta \in A} \tau^7_{\delta,\alpha} \tau^3_{\delta,\gamma,w} \quad (2r_D r_T^2 r_V) \quad (8434)$$

$$\tau^9_{\gamma,w,a} = \sum_{\alpha \in B} W^1_{a,\alpha} \tau^0_{\gamma,\alpha,w} \tau^8_{\gamma,\alpha,w} \quad (3r_D r_T r_V N_v) \quad (8435)$$

$${}^2R^3_{a,\gamma} \leftarrow \sum_{w \in D} {}^2D^3_{a,w} \tau^9_{\gamma,w,a} \quad (2r_D r_T N_v) \quad (8436)$$

Raw expression

$${}^2R^3_{b,\zeta} \leftarrow - \sum_{\gamma \in A} \sum_{i \in O} \sum_{j \in O} \sum_{k \in O} \sum_{a \in V} \sum_{c \in V} \frac{1}{2} Y^{1,*}_{a,\gamma} Y^{2,*}_{i,\gamma} Z^*_{\gamma,\zeta} Y^{4,*}_{j,\zeta} {}^2D^{a,i,b,j} {}^2T_{a,i,c,k} V_{b,c,k,j} \quad (8437)$$

Factorized expression

$$\tau^0_{\gamma,\delta,w} = \sum_{i \in O} {}^2D^4_{i,w} Y^2_{i,\gamma} Y^{4,*}_{i,\delta} \quad (3r_D r_T^2 N_o) \quad (8438)$$

$$\tau^1_{\alpha,i,j} = \sum_{\beta \in B} X_{\alpha,\beta} W^3_{i,\beta} W^4_{j,\beta} \quad (3r_V^2 N_o^2) \quad (8439)$$

$$\tau^2_{\gamma,\alpha,i} = \sum_{j \in O} Y^4_{j,\gamma} \tau^1_{\alpha,j,i} \quad (2r_T r_V N_o^2) \quad (8440)$$

$$\tau^3_{\gamma,\alpha} = \sum_{a \in V} W^2_{a,\alpha} Y^3_{a,\gamma} \quad (2r_T r_V N_v) \quad (8441)$$

$$\tau^4_{\gamma,i,a} = \sum_{\alpha \in B} W^1_{a,\alpha} \tau^3_{\gamma,\alpha} \tau^2_{\gamma,\alpha,i} \quad (3r_T r_V N_o N_v) \quad (8442)$$

$$\tau^7_{\gamma,\delta,w} = \sum_{\epsilon \in A} Z_{\epsilon,\gamma} \tau^6_{\epsilon,\delta,w} \quad (2r_D r_T^3) \quad (8455)$$

$$\tau^5_{\gamma,\delta,w} = \sum_{i \in O} \sum_{a \in V} {}^2D^1_{a,w} {}^2D^2_{i,w} Y^{1,*}_{a,\delta} Y^{2,*}_{i,\delta} \tau^4_{\gamma,i,a} \quad (5r_D r_T^2 N_o N_v) \quad (8443)$$

$${}^2R^3_{a,\gamma} \leftarrow - \sum_{\delta \in A} \sum_{w \in D} \frac{1}{2} {}^2D^3_{a,w} Y^3_{a,\delta} \tau^0_{\delta,\gamma,w} \tau^7_{\delta,\gamma,w} \quad (4r_D r_T^2 N_v) \quad (8456)$$

$$\tau^6_{\gamma,\delta,w} = \sum_{\epsilon \in A} Z^*_{\epsilon,\delta} \tau^5_{\gamma,\epsilon,w} \quad (2r_D r_T^3) \quad (8444)$$

Raw expression

$$\tau^7_{\gamma,\delta,w} = \sum_{\epsilon \in A} Z_{\gamma,\epsilon} \tau^6_{\epsilon,\delta,w} \quad (2r_D r_T^3) \quad (8445)$$

$${}^2R^3_{b,\zeta} \leftarrow - \sum_{\gamma \in A} \sum_{i \in O} \sum_{j \in O} \sum_{k \in O} \sum_{a \in V} \sum_{c \in V} \frac{1}{2} Y^{1,*}_{a,\gamma} Y^{2,*}_{i,\gamma} Z^*_{\gamma,\zeta} Y^{4,*}_{j,\zeta} {}^2D^{a,i,b,j} {}^2T_{a,k,c,j} V_{b,c,k,i} \quad (8457)$$

$${}^2R^3_{a,\gamma} \leftarrow - \sum_{\delta \in A} \sum_{w \in D} \frac{1}{2} {}^2D^3_{a,w} Y^1_{a,\delta} \tau^0_{\delta,\gamma,w} \tau^7_{\delta,\gamma,w} \quad (4r_D r_T^2 N_v) \quad (8446)$$

Factorized expression

$$\tau^0_{\gamma,\alpha,w} = \sum_{a \in V} {}^2D^1_{a,w} W^1_{a,\alpha} Y^{1,*}_{a,\gamma} \quad (3r_D r_T r_V N_v) \quad (8458)$$

Raw expression

$${}^2R^3_{b,\zeta} \leftarrow - \sum_{\gamma \in A} \sum_{i \in O} \sum_{j \in O} \sum_{k \in O} \sum_{a \in V} \sum_{c \in V} \frac{1}{2} Y^{1,*}_{a,\gamma} Y^{2,*}_{i,\gamma} Z^*_{\gamma,\zeta} Y^{4,*}_{j,\zeta} {}^2D^{a,i,b,j} {}^2T_{a,k,c,i} V_{b,j,k,c} \quad (8447)$$

$$\tau^1_{\gamma,\alpha} = \sum_{a \in V} W^2_{a,\alpha} Y^3_{a,\gamma} \quad (2r_T r_V N_v) \quad (8459)$$

Factorized expression

$$\tau^2_{\gamma,\alpha,i} = \sum_{\delta \in A} Z_{\gamma,\delta} Y^4_{i,\delta} \tau^1_{\delta,\alpha} \quad (3r_T^2 r_V N_o) \quad (8460)$$

$$\tau^0_{\gamma,\delta,w} = \sum_{i \in O} {}^2D^4_{i,w} Y^4_{i,\gamma} Y^{4,*}_{i,\delta} \quad (3r_D r_T^2 N_o) \quad (8448)$$

$$\tau^3_{\gamma,\delta,\alpha,w} = \sum_{i \in O} {}^2D^2_{i,w} Y^{2,*}_{i,\delta} \tau^0_{\delta,\alpha,w} \tau^2_{\gamma,\alpha,i} \quad (4r_D r_T^2 r_V N_o) \quad (8461)$$

$$\tau^1_{\alpha,i,j} = \sum_{\beta \in B} X_{\alpha,\beta} W^3_{i,\beta} W^4_{j,\beta} \quad (3r_V^2 N_o^2) \quad (8449)$$

$$\tau^4_{\alpha,i,j} = \sum_{\beta \in B} X_{\alpha,\beta} W^3_{i,\beta} W^4_{j,\beta} \quad (3r_V^2 N_o^2) \quad (8462)$$

$$\tau^2_{\gamma,\alpha,i} = \sum_{j \in O} Y^2_{j,\gamma} \tau^1_{\alpha,j,i} \quad (2r_T r_V N_o^2) \quad (8450)$$

$$\tau^5_{\gamma,\alpha,i} = \sum_{j \in O} Y^2_{j,\gamma} \tau^4_{\alpha,j,i} \quad (2r_T r_V N_o^2) \quad (8463)$$

$$\tau^3_{\gamma,\alpha} = \sum_{a \in V} W^2_{a,\alpha} Y^1_{a,\gamma} \quad (2r_T r_V N_v) \quad (8451)$$

$$\tau^6_{\gamma,\delta,w,i} = \sum_{\alpha \in B} \tau^5_{\gamma,\alpha,i} \tau^3_{\gamma,\delta,\alpha,w} \quad (2r_D r_T^2 r_V N_o) \quad (8464)$$

$$\tau^4_{\gamma,i,a} = \sum_{\alpha \in B} W^1_{a,\alpha} \tau^3_{\gamma,\alpha} \tau^2_{\gamma,\alpha,i} \quad (3r_T r_V N_o N_v) \quad (8452)$$

$$\tau^7_{\gamma,\delta,w} = \sum_{\epsilon \in A} \sum_{i \in O} {}^2D^4_{i,w} Z^*_{\epsilon,\delta} Y^{4,*}_{i,\delta} \tau^6_{\gamma,\epsilon,w,i} \quad (4r_D r_T^3 N_o) \quad (8465)$$

$$\tau^5_{\gamma,\delta,w} = \sum_{i \in O} \sum_{a \in V} {}^2D^1_{a,w} {}^2D^2_{i,w} Y^{1,*}_{a,\delta} Y^{2,*}_{i,\delta} \tau^4_{\gamma,i,a} \quad (5r_D r_T^2 N_o N_v) \quad (8453)$$

$$\tau^6_{\gamma,\delta,w} = \sum_{\epsilon \in A} Z^*_{\epsilon,\delta} \tau^5_{\gamma,\epsilon,w} \quad (2r_D r_T^3) \quad (8454)$$

$${}^2R^3_{a,\gamma} \leftarrow - \sum_{\delta \in A} \sum_{w \in D} \frac{1}{2} {}^2D^3_{a,w} Y^1_{a,\delta} \tau^7_{\delta,\gamma,w} \quad (3r_D r_T^2 N_v) \quad (8466)$$

Raw expression

$${}^2R^3_{b,\zeta} \leftarrow - \sum_{\gamma \in A} \sum_{i \in O} \sum_{j \in O} \sum_{k \in O} \sum_{a \in V} \sum_{c \in V} \frac{1}{2} Y^{1,*}_{a,\gamma} Y^{2,*}_{i,\gamma} Z^*_{\gamma,\zeta} Y^{4,*}_{j,\zeta} {}^2D^{a,i,b,j} {}^2T_{b,j,c,k} V_{a,c,k,i} \quad (8467)$$

Factorized expression

$$\tau^0_{\gamma,\alpha,w} = \sum_{a \in V} {}^2D^1_{a,w} W^1_{a,\alpha} Y^{1,*}_{a,\gamma} \quad (3r_D r_T r_V N_v) \quad (8468)$$

$$\tau^1_{\gamma,\alpha} = \sum_{a \in V} W^2_{a,\alpha} Y^1_{a,\gamma} \quad (2r_T r_V N_v) \quad (8469)$$

$$\tau^2_{\gamma,\alpha,i} = \sum_{\delta \in A} Y^2_{i,\delta} Z_{\delta,\gamma} \tau^1_{\delta,\alpha} \quad (3r_T^2 r_V N_o) \quad (8470)$$

$$\tau^3_{\gamma,\delta,\alpha,w} = \sum_{i \in O} {}^2D^2_{i,w} Y^{2,*}_{i,\delta} \tau^0_{\delta,\alpha,w} \tau^2_{\gamma,\alpha,i} \quad (4r_D r_T^2 r_V N_o) \quad (8471)$$

$$\tau^4_{\alpha,i,j} = \sum_{\beta \in B} X_{\alpha,\beta} W^3_{i,\beta} W^4_{j,\beta} \quad (3r_V^2 N_o^2) \quad (8472)$$

$$\tau^5_{\gamma,\alpha,i} = \sum_{j \in O} Y^4_{j,\gamma} \tau^4_{\alpha,j,i} \quad (2r_T r_V N_o^2) \quad (8473)$$

$$\tau^6_{\gamma,\delta,w,i} = \sum_{\alpha \in B} \tau^5_{\gamma,\alpha,i} \tau^3_{\gamma,\delta,\alpha,w} \quad (2r_D r_T^2 r_V N_o) \quad (8474)$$

$$\tau^7_{\gamma,\delta,w} = \sum_{\epsilon \in A} \sum_{i \in O} {}^2D^4_{i,w} Z^*_{\epsilon,\delta} Y^{4,*}_{i,\delta} \tau^6_{\gamma,\epsilon,w,i} \quad (4r_D r_T^3 N_o) \quad (8475)$$

$${}^2R^3_{a,\gamma} \leftarrow - \sum_{\delta \in A} \sum_{w \in D} \frac{1}{2} {}^2D^3_{a,w} Y^3_{a,\delta} \tau^7_{\delta,\gamma,w} \quad (3r_D r_T^2 N_v) \quad (8476)$$

Raw expression

$${}^2R^3_{b,\zeta} \leftarrow - \sum_{\gamma \in A} \sum_{i \in O} \sum_{j \in O} \sum_{k \in O} \sum_{a \in V} \sum_{c \in V} \frac{1}{2} Y^{1,*}_{a,\gamma} Y^{2,*}_{i,\gamma} Z^*_{\gamma,\zeta} Y^{4,*}_{j,\zeta} {}^2D^{a,i,b,j} {}^2T_{b,k,c,i} V_{a,c,k,j} \quad (8477)$$

Factorized expression

$$\tau^0_{\gamma,\alpha} = \sum_{i \in O} W^3_{i,\alpha} Y^2_{i,\gamma} \quad (2r_T r_V N_o) \quad (8478)$$

$$\tau^1_{\gamma,\alpha} = \sum_{a \in V} W^4_{a,\alpha} Y^3_{a,\gamma} \quad (2r_T r_V N_v) \quad (8479)$$

$$\tau^2_{\gamma,\alpha,i} = \sum_{\delta \in A} Z_{\gamma,\delta} Y^4_{i,\delta} \tau^1_{\delta,\alpha} \quad (3r_T^2 r_V N_o) \quad (8480)$$

$$\tau^3_{\gamma,\alpha,w} = \sum_{a \in V} {}^2D^1_{a,w} W^1_{a,\alpha} Y^{1,*}_{a,\gamma} \quad (3r_D r_T r_V N_v) \quad (8481)$$

$$\tau^4_{\gamma,\alpha,w} = \sum_{i \in O} {}^2D^2_{i,w} W^2_{i,\alpha} Y^{2,*}_{i,\gamma} \quad (3r_D r_T r_V N_o) \quad (8482)$$

$$\tau^5_{\gamma,\alpha,w} = \sum_{\beta \in B} X_{\beta,\alpha} \tau^3_{\gamma,\beta,w} \tau^4_{\gamma,\beta,w} \quad (3r_D r_T r_V^2) \quad (8483)$$

$$\tau^6_{\gamma,\alpha,w} = \sum_{\delta \in A} Z^*_{\delta,\gamma} \tau^5_{\delta,\alpha,w} \quad (2r_D r_T^2 r_V) \quad (8484)$$

$$\tau^7_{\gamma,\delta,w,i} = \sum_{\alpha \in B} \tau^0_{\gamma,\alpha} \tau^2_{\gamma,\alpha,i} \tau^6_{\delta,\alpha,w} \quad (3r_D r_T^2 r_V N_o) \quad (8485)$$

$$\tau^8_{\gamma,\delta,w} = \sum_{i \in O} {}^2D^4_{i,w} Y^{4,*}_{i,\delta} \tau^7_{\gamma,\delta,w,i} \quad (3r_D r_T^2 N_o) \quad (8486)$$

$${}^2R^3_{a,\gamma} \leftarrow - \sum_{\delta \in A} \sum_{w \in D} \frac{1}{2} {}^2D^3_{a,w} Y^1_{a,\delta} \tau^8_{\delta,\gamma,w} \quad (3r_D r_T^2 N_v) \quad (8487)$$

Raw expression

$${}^2R^3_{b,\zeta} \leftarrow - \sum_{\gamma \in A} \sum_{i \in O} \sum_{j \in O} \sum_{k \in O} \sum_{a \in V} \sum_{c \in V} \frac{1}{2} Y^{1,*}_{a,\gamma} Y^{2,*}_{i,\gamma} Z^*_{\gamma,\zeta} Y^{4,*}_{j,\zeta} {}^2D^{a,i,b,j} {}^2T_{b,k,c,j} V_{a,i,k,c} \quad (8488)$$

Factorized expression

$$\tau^0_{\gamma,\alpha} = \sum_{a \in V} W^4_{a,\alpha} Y^1_{a,\gamma} \quad (2r_T r_V N_v) \quad (8489)$$

$$\tau^1_{\gamma,\alpha,i} = \sum_{\delta \in A} Y^2_{i,\delta} Z_{\delta,\gamma} \tau^0_{\delta,\alpha} \quad (3r_T^2 r_V N_o) \quad (8490)$$

$$\tau^2_{\gamma,\alpha} = \sum_{i \in O} W^3_{i,\alpha} Y^4_{i,\gamma} \quad (2r_T r_V N_o) \quad (8491)$$

$$\tau^3_{\gamma,\alpha,w} = \sum_{a \in V} {}^2D^1_{a,w} W^1_{a,\alpha} Y^{1,*}_{a,\gamma} \quad (3r_D r_T r_V N_v) \quad (8492)$$

$$\tau^4_{\gamma,\alpha,w} = \sum_{i \in O} {}^2D^2_{i,w} W^2_{i,\alpha} Y^{2,*}_{i,\gamma} \quad (3r_D r_T r_V N_o) \quad (8493)$$

$$\tau^5_{\gamma,\alpha,w} = \sum_{\beta \in B} X_{\beta,\alpha} \tau^3_{\gamma,\beta,w} \tau^4_{\gamma,\beta,w} \quad (3r_D r_T r_V^2) \quad (8494)$$

$$\tau^6_{\gamma,\alpha,w} = \sum_{\delta \in A} Z^*_{\delta,\gamma} \tau^5_{\delta,\alpha,w} \quad (2r_D r_T^2 r_V) \quad (8495)$$

$$\tau^7_{\gamma,\delta,w,i} = \sum_{\alpha \in B} \tau^2_{\gamma,\alpha} \tau^1_{\gamma,\alpha,i} \tau^6_{\delta,\alpha,w} \quad (3r_D r_T^2 r_V N_o) \quad (8496)$$

$$\tau^8_{\gamma,\delta,w} = \sum_{i \in O} {}^2D^4_{i,w} Y^{4,*}_{i,\delta} \tau^7_{\gamma,\delta,w,i} \quad (3r_D r_T^2 N_o) \quad (8497)$$

$${}^2R^3_{a,\gamma} \leftarrow - \sum_{\delta \in A} \sum_{w \in D} \frac{1}{2} {}^2D^3_{a,w} Y^3_{a,\delta} \tau^8_{\delta,\gamma,w} \quad (3r_D r_T^2 N_v) \quad (8498)$$

Raw expression

$${}^2R^3_{b,\zeta} \leftarrow - \sum_{\gamma \in A} \sum_{i \in O} \sum_{j \in O} \sum_{k \in O} \sum_{a \in V} \sum_{c \in V} \frac{1}{2} Y^{1,*}_{a,\gamma} Y^{2,*}_{i,\gamma} Z^*_{\gamma,\zeta} Y^{4,*}_{j,\zeta} {}^2D^{a,i,b,j}_{c,i,a,k} T_{c,i,a,k} V_{b,j,k,c} \quad (8499)$$

Factorized expression

$$\tau^0_{\gamma,\alpha} = \sum_{a \in V} W^2_{a,\alpha} Y^3_{a,\gamma} \quad (2r_T r_V N_v) \quad (8500)$$

$$\tau^1_{\gamma,\alpha,i} = \sum_{\delta \in A} Z_{\gamma,\delta} Y^4_{i,\delta} \tau^0_{\delta,\alpha} \quad (3r_T^2 r_V N_o) \quad (8501)$$

$$\tau^2_{\gamma,\delta,w} = \sum_{a \in V} {}^2D^1_{a,w} Y^1_{a,\gamma} Y^{1,*}_{a,\delta} \quad (3r_D r_T^2 N_v) \quad (8502)$$

$$\tau^3_{\gamma,\delta,w,i} = \sum_{\epsilon \in A} {}^2D^2_{i,w} Y^{2,*}_{i,\epsilon} Z^*_{\epsilon,\delta} \tau^2_{\gamma,\epsilon,w} \quad (4r_D r_T^3 N_o) \quad (8503)$$

$$\tau^4_{\alpha,i,j} = \sum_{\beta \in B} X_{\alpha,\beta} W^3_{i,\beta} W^4_{j,\beta} \quad (3r_V^2 N_o^2) \quad (8504)$$

$$\tau^5_{\gamma,\alpha,i} = \sum_{j \in O} Y^2_{j,\gamma} \tau^4_{\alpha,j,i} \quad (2r_T r_V N_o^2) \quad (8505)$$

$$\tau^6_{\gamma,\delta,\alpha,w} = \sum_{i \in O} \tau^5_{\gamma,\alpha,i} \tau^3_{\gamma,\delta,w,i} \quad (2r_D r_T^2 r_V N_o) \quad (8506)$$

$$\tau^7_{\gamma,\alpha,w,i} = \sum_{\delta \in A} \tau^1_{\delta,\alpha,i} \tau^6_{\delta,\gamma,\alpha,w} \quad (2r_D r_T^2 r_V N_o) \quad (8507)$$

$$\tau^8_{\gamma,\alpha,w} = \sum_{i \in O} {}^2D^4_{i,w} Y^{4,*}_{i,\gamma} \tau^7_{\gamma,\alpha,w,i} \quad (3r_D r_T r_V N_o) \quad (8508)$$

$$\tau^9_{\gamma,w,a} = \sum_{\alpha \in B} W^1_{a,\alpha} \tau^8_{\gamma,\alpha,w} \quad (2r_D r_T r_V N_v) \quad (8509)$$

$${}^2R^3_{a,\gamma} \leftarrow - \sum_{w \in D} \frac{1}{2} {}^2D^3_{a,w} \tau^9_{\gamma,w,a} \quad (2r_D r_T N_v) \quad (8510)$$

Raw expression

$${}^2R^3_{b,\zeta} \leftarrow - \sum_{\gamma \in A} \sum_{i \in O} \sum_{j \in O} \sum_{k \in O} \sum_{a \in V} \sum_{c \in V} \frac{1}{2} Y^{1,*}_{a,\gamma} Y^{2,*}_{i,\gamma} Z^*_{\gamma,\zeta} Y^{4,*}_{j,\zeta} {}^2D^{a,i,b,j}_{c,i,b,k} T_{c,i,b,k} V_{a,c,k,j} \quad (8511)$$

Factorized expression

$$\tau^0_{\gamma,\delta,w} = \sum_{a \in V} {}^2D^1_{a,w} Y^3_{a,\gamma} Y^{1,*}_{a,\delta} \quad (3r_D r_T^2 N_v) \quad (8512)$$

$$\tau^1_{\gamma,\delta,w,i} = \sum_{\epsilon \in A} {}^2D^2_{i,w} Y^{2,*}_{i,\epsilon} Z^*_{\epsilon,\delta} \tau^0_{\gamma,\epsilon,w} \quad (4r_D r_T^3 N_o) \quad (8513)$$

$$\tau^2_{\alpha,i,j} = \sum_{\beta \in B} X_{\alpha,\beta} W^3_{i,\beta} W^4_{j,\beta} \quad (3r_V^2 N_o^2) \quad (8514)$$

$$\tau^3_{\gamma,\alpha,i} = \sum_{j \in O} Y^4_{j,\gamma} \tau^2_{\alpha,j,i} \quad (2r_T r_V N_o^2) \quad (8515)$$

$$\tau^4_{\alpha,i,j} = \sum_{\beta \in B} X_{\alpha,\beta} W^3_{i,\beta} W^4_{j,\beta} \quad (3r_V^2 N_o^2) \quad (8528)$$

$$\tau^4_{\gamma,\delta,\alpha,w} = \sum_{i \in O} \tau^3_{\gamma,\alpha,i} \tau^1_{\gamma,\delta,w,i} \quad (2r_D r_T^2 r_V N_o) \quad (8516)$$

$$\tau^5_{\gamma,\alpha,i} = \sum_{j \in O} Y^4_{j,\gamma} \tau^4_{\alpha,j,i} \quad (2r_T r_V N_o^2) \quad (8529)$$

$$\tau^5_{\gamma,\alpha} = \sum_{a \in V} W^2_{a,\alpha} Y^1_{a,\gamma} \quad (2r_T r_V N_v) \quad (8517)$$

$$\tau^6_{\gamma,\alpha} = \sum_{a \in V} W^2_{a,\alpha} Y^3_{a,\gamma} \quad (2r_T r_V N_v) \quad (8530)$$

$$\tau^6_{\gamma,\alpha,i} = \sum_{\delta \in A} Y^2_{i,\delta} Z_{\delta,\gamma} \tau^5_{\delta,\alpha} \quad (3r_T^2 r_V N_o) \quad (8518)$$

$$\tau^7_{\gamma,i,a} = \sum_{\alpha \in B} W^1_{a,\alpha} \tau^6_{\gamma,\alpha} \tau^5_{\gamma,\alpha,i} \quad (3r_T r_V N_o N_v) \quad (8531)$$

$$\tau^7_{\gamma,\alpha,w,i} = \sum_{\delta \in A} \tau^6_{\delta,\alpha,i} \tau^4_{\delta,\gamma,\alpha,w} \quad (2r_D r_T^2 r_V N_o) \quad (8519)$$

$$\tau^8_{\gamma,w,a} = \sum_{\delta \in A} \sum_{i \in O} {}^2D^4_{i,w} Y^{4,*}_{i,\gamma} \tau^3_{\delta,\gamma,w} \tau^7_{\delta,i,a} \quad (4r_D r_T^2 N_o N_v) \quad (8532)$$

$$\tau^8_{\gamma,\alpha,w} = \sum_{i \in O} {}^2D^4_{i,w} Y^{4,*}_{i,\gamma} \tau^7_{\gamma,\alpha,w,i} \quad (3r_D r_T r_V N_o) \quad (8520)$$

$${}^2R^3_{a,\gamma} \leftarrow - \sum_{w \in D} \frac{1}{2} {}^2D^3_{a,w} \tau^8_{\gamma,w,a} \quad (2r_D r_T N_v) \quad (8533)$$

Raw expression

$$\tau^9_{\gamma,w,a} = \sum_{\alpha \in B} W^1_{a,\alpha} \tau^8_{\gamma,\alpha,w} \quad (2r_D r_T r_V N_v) \quad (8521)$$

$${}^2R^3_{a,\gamma} \leftarrow - \sum_{w \in D} \frac{1}{2} {}^2D^3_{a,w} \tau^9_{\gamma,w,a} \quad (2r_D r_T N_v) \quad (8522)$$

$${}^2R^3_{b,\zeta} \leftarrow - \sum_{\gamma \in A} \sum_{i \in O} \sum_{j \in O} \sum_{k \in O} \sum_{a \in V} \sum_{c \in V} \frac{1}{2} Y^{1,*}_{a,\gamma} Y^{2,*}_{i,\gamma} Z^*_{\gamma,\zeta} Y^{4,*}_{j,\zeta} {}^2D^{a,i,b,j} {}^2T_{c,j,b,k} V_{a,i,k,c} \quad (8534)$$

Raw expression

$${}^2R^3_{b,\zeta} \leftarrow - \sum_{\gamma \in A} \sum_{i \in O} \sum_{j \in O} \sum_{k \in O} \sum_{a \in V} \sum_{c \in V} \frac{1}{2} Y^{1,*}_{a,\gamma} Y^{2,*}_{i,\gamma} Z^*_{\gamma,\zeta} Y^{4,*}_{j,\zeta} {}^2D^{a,i,b,j} {}^2T_{c,j,a,k} V_{b,c,k,i} \quad (8523)$$

Factorized expression

$$\tau^0_{\gamma,\delta,w} = \sum_{a \in V} {}^2D^1_{a,w} Y^3_{a,\gamma} Y^{1,*}_{a,\delta} \quad (3r_D r_T^2 N_v) \quad (8535)$$

$$\tau^1_{\gamma,\delta,w} = \sum_{i \in O} {}^2D^2_{i,w} Y^4_{i,\gamma} Y^{2,*}_{i,\delta} \quad (3r_D r_T^2 N_o) \quad (8536)$$

$$\tau^0_{\gamma,\delta,w} = \sum_{a \in V} {}^2D^1_{a,w} Y^1_{a,\gamma} Y^{1,*}_{a,\delta} \quad (3r_D r_T^2 N_v) \quad (8524)$$

$$\tau^2_{\gamma,\delta,w} = \sum_{\epsilon \in A} Z^*_{\epsilon,\delta} \tau^0_{\gamma,\epsilon,w} \tau^1_{\gamma,\epsilon,w} \quad (3r_D r_T^3) \quad (8537)$$

$$\tau^1_{\gamma,\delta,w} = \sum_{i \in O} {}^2D^2_{i,w} Y^2_{i,\gamma} Y^{2,*}_{i,\delta} \quad (3r_D r_T^2 N_o) \quad (8525)$$

$$\tau^3_{\gamma,\delta,w} = \sum_{\epsilon \in A} Z_{\gamma,\epsilon} \tau^2_{\epsilon,\delta,w} \quad (2r_D r_T^3) \quad (8538)$$

$$\tau^2_{\gamma,\delta,w} = \sum_{\epsilon \in A} Z^*_{\epsilon,\delta} \tau^0_{\gamma,\epsilon,w} \tau^1_{\gamma,\epsilon,w} \quad (3r_D r_T^3) \quad (8526)$$

$$\tau^4_{\alpha,i,j} = \sum_{\beta \in B} X_{\alpha,\beta} W^3_{i,\beta} W^4_{j,\beta} \quad (3r_V^2 N_o^2) \quad (8539)$$

$$\tau^3_{\gamma,\delta,w} = \sum_{\epsilon \in A} Z_{\gamma,\epsilon} \tau^2_{\epsilon,\delta,w} \quad (2r_D r_T^3) \quad (8527)$$

$$\tau^5_{\gamma,\alpha,i} = \sum_{j \in O} Y^2_{j,\gamma} \tau^4_{\alpha,j,i} \quad (2r_T r_V N_o^2) \quad (8540)$$

$$\tau_{\gamma,\alpha}^6 = \sum_{a \in V} W_{a,\alpha}^2 Y_{a,\gamma}^1 \quad (2r_T r_V N_v) \quad (8541)$$

$$\tau_{\gamma,w,a}^8 = \sum_{\alpha \in B} W_{a,\alpha}^1 \tau_{\gamma,\alpha,w}^0 \tau_{\gamma,\alpha,w}^7 \quad (3r_D r_T r_V N_v) \quad (8554)$$

$$\tau_{\gamma,i,a}^7 = \sum_{\alpha \in B} W_{a,\alpha}^1 \tau_{\gamma,\alpha}^6 \tau_{\gamma,\alpha,i}^5 \quad (3r_T r_V N_o N_v) \quad (8542)$$

$${}^2R_{a,\gamma}^3 \leftarrow - \sum_{w \in D} \frac{1}{2} {}^2D_{a,w}^3 \tau_{\gamma,w,a}^8 \quad (2r_D r_T N_v) \quad (8555)$$

$$\tau_{\gamma,w,a}^8 = \sum_{\delta \in A} \sum_{i \in O} {}^2D_{i,w}^4 Y_{i,\gamma}^{4,*} \tau_{\delta,\gamma,w}^3 \tau_{\delta,i,a}^7 \quad (4r_D r_T^2 N_o N_v) \quad (8543)$$

Raw expression

$${}^2R_{a,\gamma}^3 \leftarrow - \sum_{w \in D} \frac{1}{2} {}^2D_{a,w}^3 \tau_{\gamma,w,a}^8 \quad (2r_D r_T N_v) \quad (8544)$$

$${}^2R_{b,\zeta}^3 \leftarrow - \sum_{\gamma \in A} \sum_{i \in O} \sum_{j \in O} \sum_{k \in O} \sum_{a \in V} \sum_{c \in V} \frac{1}{2} Y_{a,\gamma}^{1,*} Y_{i,\gamma}^{2,*} Z_{\gamma,\zeta}^* Y_{j,\zeta}^{4,*} {}^2D_{a,i,b,j} {}^2T_{c,k,b,j} V_{a,c,k,i} \quad (8556)$$

Raw expression

$${}^2R_{b,\zeta}^3 \leftarrow - \sum_{\gamma \in A} \sum_{i \in O} \sum_{j \in O} \sum_{k \in O} \sum_{a \in V} \sum_{c \in V} \frac{1}{2} Y_{a,\gamma}^{1,*} Y_{i,\gamma}^{2,*} Z_{\gamma,\zeta}^* Y_{j,\zeta}^{4,*} {}^2D_{a,i,b,j} {}^2T_{c,k,a,i} V_{b,c,k,j} \quad (8545)$$

Factorized expression

$$\tau_{\gamma,\alpha,w}^0 = \sum_{i \in O} {}^2D_{i,w}^4 W_{i,\alpha}^2 Y_{i,\gamma}^{4,*} \quad (3r_D r_T r_V N_o) \quad (8557)$$

Factorized expression

$$\tau_{\gamma,\alpha,w}^0 = \sum_{i \in O} {}^2D_{i,w}^4 W_{i,\alpha}^2 Y_{i,\gamma}^{4,*} \quad (3r_D r_T r_V N_o) \quad (8546)$$

$$\tau_{\gamma,\delta,w}^1 = \sum_{a \in V} {}^2D_{a,w}^1 Y_{a,\gamma}^3 Y_{a,\delta}^{1,*} \quad (3r_D r_T^2 N_v) \quad (8558)$$

$$\tau_{\gamma,\delta,w}^1 = \sum_{a \in V} {}^2D_{a,w}^1 Y_{a,\gamma}^1 Y_{a,\delta}^{1,*} \quad (3r_D r_T^2 N_v) \quad (8547)$$

$$\tau_{\gamma,\alpha}^2 = \sum_{a \in V} W_{a,\alpha}^4 Y_{a,\gamma}^1 \quad (2r_T r_V N_v) \quad (8559)$$

$$\tau_{\gamma,\alpha,i}^3 = \sum_{\delta \in A} Y_{i,\delta}^2 Z_{\delta,\gamma} \tau_{\delta,\alpha}^2 \quad (3r_T^2 r_V N_o) \quad (8560)$$

$$\tau_{\gamma,\alpha}^2 = \sum_{i \in O} W_{i,\alpha}^3 Y_{i,\gamma}^2 \quad (2r_T r_V N_o) \quad (8548)$$

$$\tau_{\gamma,\alpha}^4 = \sum_{i \in O} W_{i,\alpha}^3 Y_{i,\gamma}^4 \quad (2r_T r_V N_o) \quad (8561)$$

$$\tau_{\gamma,\alpha}^3 = \sum_{a \in V} W_{a,\alpha}^4 Y_{a,\gamma}^3 \quad (2r_T r_V N_v) \quad (8549)$$

$$\tau_{\gamma,\alpha,w}^5 = \sum_{\delta \in A} \sum_{i \in O} {}^2D_{i,w}^2 Y_{i,\gamma}^{2,*} \tau_{\delta,\alpha}^4 \tau_{\delta,\gamma,w}^1 \tau_{\delta,\alpha,i}^3 \quad (5r_D r_T^2 r_V N_o) \quad (8562)$$

$$\tau_{\gamma,\alpha,i}^4 = \sum_{\delta \in A} Z_{\gamma,\delta} Y_{i,\delta}^4 \tau_{\delta,\alpha}^3 \quad (3r_T^2 r_V N_o) \quad (8550)$$

$$\tau_{\gamma,\alpha,w}^5 = \sum_{\delta \in A} \sum_{i \in O} {}^2D_{i,w}^2 Y_{i,\gamma}^{2,*} \tau_{\delta,\alpha}^2 \tau_{\delta,\gamma,w}^1 \tau_{\delta,\alpha,i}^4 \quad (5r_D r_T^2 r_V N_o) \quad (8551)$$

$$\tau_{\gamma,\alpha,w}^6 = \sum_{\beta \in B} X_{\alpha,\beta} \tau_{\gamma,\beta,w}^5 \quad (2r_D r_T r_V^2) \quad (8563)$$

$$\tau_{\gamma,\alpha,w}^6 = \sum_{\beta \in B} X_{\alpha,\beta} \tau_{\gamma,\beta,w}^5 \quad (2r_D r_T r_V^2) \quad (8552)$$

$$\tau_{\gamma,\alpha,w}^7 = \sum_{\delta \in A} Z_{\delta,\gamma}^* \tau_{\delta,\alpha,w}^6 \quad (2r_D r_T^2 r_V) \quad (8564)$$

$$\tau_{\gamma,\alpha,w}^7 = \sum_{\delta \in A} Z_{\delta,\gamma}^* \tau_{\delta,\alpha,w}^6 \quad (2r_D r_T^2 r_V) \quad (8553)$$

$$\tau_{\gamma,w,a}^8 = \sum_{\alpha \in B} W_{a,\alpha}^1 \tau_{\gamma,\alpha,w}^0 \tau_{\gamma,\alpha,w}^7 \quad (3r_D r_T r_V N_v) \quad (8565)$$



$${}^2R^3_{a,\gamma} \leftarrow - \sum_{w \in D} \frac{1}{2} {}^2D^3_{a,w} \tau^8_{\gamma,w,a} \quad (2r_D r_T N_v) \quad (8566)$$

Raw expression

$${}^2R^3_{b,\zeta} \leftarrow \sum_{\gamma \in A} \sum_{i \in O} \sum_{j \in O} \sum_{a \in V} \sum_{c \in V} \frac{1}{2} Y^{1,*}_{a,\gamma} Y^{2,*}_{i,\gamma} Z^*_{\gamma,\zeta} Y^{4,*}_{j,\zeta} f_{a,c} {}^2D^{a,i,b,j} {}^2T_{b,j,c,i} \quad (8567)$$

Factorized expression

$$\tau^0_{\gamma,i} = \sum_{j \in O} Y^4_{j,\gamma} f_{j,i} \quad (2r_T N_o^2) \quad (8568)$$

$$\tau^1_{\gamma,\delta,w} = \sum_{i \in O} {}^2D^4_{i,w} Y^{4,*}_{i,\delta} \tau^0_{\gamma,i} \quad (3r_D r_T^2 N_o) \quad (8569)$$

$$\tau^2_{\gamma,\delta,w} = \sum_{a \in V} {}^2D^1_{a,w} Y^1_{a,\gamma} Y^{1,*}_{a,\delta} \quad (3r_D r_T^2 N_v) \quad (8570)$$

$$\tau^3_{\gamma,\delta,w} = \sum_{i \in O} {}^2D^2_{i,w} Y^2_{i,\gamma} Y^{2,*}_{i,\delta} \quad (3r_D r_T^2 N_o) \quad (8571)$$

$$\tau^4_{\gamma,\delta,w} = \sum_{\epsilon \in A} Z^*_{\epsilon,\delta} \tau^2_{\gamma,\epsilon,w} \tau^3_{\gamma,\epsilon,w} \quad (3r_D r_T^3) \quad (8572)$$

$$\tau^5_{\gamma,\delta,w} = \sum_{\epsilon \in A} Z_{\epsilon,\gamma} \tau^4_{\epsilon,\delta,w} \quad (2r_D r_T^3) \quad (8573)$$

$${}^2R^3_{a,\gamma} \leftarrow - \sum_{\delta \in A} \sum_{w \in D} \frac{1}{2} {}^2D^3_{a,w} Y^3_{a,\delta} \tau^1_{\delta,\gamma,w} \tau^5_{\delta,\gamma,w} \quad (4r_D r_T^2 N_v) \quad (8574)$$

Raw expression

$${}^2R^3_{b,\zeta} \leftarrow \sum_{\gamma \in A} \sum_{i \in O} \sum_{j \in O} \sum_{a \in V} \sum_{c \in V} \frac{1}{2} Y^{1,*}_{a,\gamma} Y^{2,*}_{i,\gamma} Z^*_{\gamma,\zeta} Y^{4,*}_{j,\zeta} f_{a,c} {}^2D^{a,i,b,j} {}^2T_{c,i,b,j} \quad (8575)$$

Factorized expression

$$\tau^0_{\gamma,\delta,w} = \sum_{i \in O} {}^2D^4_{i,w} Y^4_{i,\gamma} Y^{4,*}_{i,\delta} \quad (3r_D r_T^2 N_o) \quad (8576)$$

$$\tau^1_{\gamma,\delta,w} = \sum_{a \in V} {}^2D^1_{a,w} Y^1_{a,\gamma} Y^{1,*}_{a,\delta} \quad (3r_D r_T^2 N_v) \quad (8577)$$

$$\tau^2_{\gamma,i} = \sum_{j \in O} Y^2_{j,\gamma} f_{j,i} \quad (2r_T N_o^2) \quad (8578)$$

$$\tau^3_{\gamma,\delta,w} = \sum_{i \in O} {}^2D^2_{i,w} Y^{2,*}_{i,\delta} \tau^2_{\gamma,i} \quad (3r_D r_T^2 N_o) \quad (8579)$$

$$\tau^4_{\gamma,\delta,w} = \sum_{\epsilon \in A} Z^*_{\epsilon,\delta} \tau^1_{\gamma,\epsilon,w} \tau^3_{\gamma,\epsilon,w} \quad (3r_D r_T^3) \quad (8580)$$

$$\tau^5_{\gamma,\delta,w} = \sum_{\epsilon \in A} Z_{\epsilon,\gamma} \tau^4_{\epsilon,\delta,w} \quad (2r_D r_T^3) \quad (8581)$$

$${}^2R^3_{a,\gamma} \leftarrow - \sum_{\delta \in A} \sum_{w \in D} \frac{1}{2} {}^2D^3_{a,w} Y^3_{a,\delta} \tau^0_{\delta,\gamma,w} \tau^5_{\delta,\gamma,w} \quad (4r_D r_T^2 N_v) \quad (8582)$$

Raw expression

$${}^2R^3_{b,\zeta} \leftarrow \sum_{\gamma \in A} \sum_{i \in O} \sum_{j \in O} \sum_{a \in V} \sum_{c \in V} \frac{1}{2} Y^{1,*}_{a,\gamma} Y^{2,*}_{i,\gamma} Z^*_{\gamma,\zeta} Y^{4,*}_{j,\zeta} f_{b,c} {}^2D^{a,i,b,j} {}^2T_{a,i,c,j} \quad (8583)$$

Factorized expression

$$\tau^0_{\gamma,\delta,w} = \sum_{i \in O} {}^2D^4_{i,w} Y^2_{i,\gamma} Y^{4,*}_{i,\delta} \quad (3r_D r_T^2 N_o) \quad (8584)$$

$$\tau^1_{\gamma,\delta,w} = \sum_{a \in V} {}^2D^1_{a,w} Y^3_{a,\gamma} Y^{1,*}_{a,\delta} \quad (3r_D r_T^2 N_v) \quad (8585)$$

$$\tau^2_{\gamma,i} = \sum_{j \in O} Y^4_{j,\gamma} f_{j,i} \quad (2r_T N_o^2) \quad (8586)$$

$$\tau^3_{\gamma,\delta,w} = \sum_{i \in O} {}^2D^2_{i,w} Y^{2,*}_{i,\delta} \tau^2_{\gamma,i} \quad (3r_D r_T^2 N_o) \quad (8587)$$

$$\tau^4_{\gamma,\delta,w} = \sum_{\epsilon \in A} Z^*_{\epsilon,\delta} \tau^1_{\gamma,\epsilon,w} \tau^3_{\gamma,\epsilon,w} \quad (3r_D r_T^3) \quad (8588)$$

$$\tau^5_{\gamma,\delta,w} = \sum_{\epsilon \in A} Z_{\gamma,\epsilon} \tau^4_{\epsilon,\delta,w} \quad (2r_D r_T^3) \quad (8589)$$

$${}^2R^3_{a,\gamma} \leftarrow - \sum_{\delta \in A} \sum_{w \in D} \frac{1}{2} {}^2D^3_{a,w} Y^1_{a,\delta} \tau^0_{\delta,\gamma,w} \tau^5_{\delta,\gamma,w} \quad (4r_D r_T^2 N_v) \quad (8590)$$

Raw expression

$${}^2R^3_{b,\zeta} \leftarrow \sum_{\gamma \in A} \sum_{i \in O} \sum_{j \in O} \sum_{a \in V} \sum_{c \in V} \frac{1}{2} Y^{1,*}_{a,\gamma} Y^{2,*}_{i,\gamma} Z^*_{\gamma,\zeta} Y^{4,*}_{j,\zeta} f_{b,c} {}^2D^{a,i,b,j} {}^2T_{c,j,a,i} \quad (8591)$$

Factorized expression

$$\tau^0_{\gamma,i} = \sum_{j \in O} Y^2_{j,\gamma} f_{j,i} \quad (2r_T N_o^2) \quad (8592)$$

$$\tau^1_{\gamma,\delta,w} = \sum_{i \in O} {}^2D^4_{i,w} Y^{4,*}_{i,\delta} \tau^0_{\gamma,i} \quad (3r_D r_T^2 N_o) \quad (8593)$$

$$\tau^2_{\gamma,\delta,w} = \sum_{a \in V} {}^2D^1_{a,w} Y^3_{a,\gamma} Y^{1,*}_{a,\delta} \quad (3r_D r_T^2 N_v) \quad (8594)$$

$$\tau^3_{\gamma,\delta,w} = \sum_{i \in O} {}^2D^2_{i,w} Y^4_{i,\gamma} Y^{2,*}_{i,\delta} \quad (3r_D r_T^2 N_o) \quad (8595)$$

$$\tau^4_{\gamma,\delta,w} = \sum_{\epsilon \in A} Z^*_{\epsilon,\delta} \tau^2_{\gamma,\epsilon,w} \tau^3_{\gamma,\epsilon,w} \quad (3r_D r_T^3) \quad (8596)$$

$$\tau^5_{\gamma,\delta,w} = \sum_{\epsilon \in A} Z_{\gamma,\epsilon} \tau^4_{\epsilon,\delta,w} \quad (2r_D r_T^3) \quad (8597)$$

$${}^2R^3_{a,\gamma} \leftarrow - \sum_{\delta \in A} \sum_{w \in D} \frac{1}{2} {}^2D^3_{a,w} Y^1_{a,\delta} \tau^1_{\delta,\gamma,w} \tau^5_{\delta,\gamma,w} \quad (4r_D r_T^2 N_v) \quad (8598)$$

Raw expression

$${}^2R^3_{b,\zeta} \leftarrow \sum_{\gamma \in A} \sum_{i \in O} \sum_{j \in O} \sum_{k \in O} \sum_{l \in O} \sum_{a \in V} \frac{1}{2} Y^{1,*}_{a,\gamma} Y^{2,*}_{i,\gamma} Z^*_{\gamma,\zeta} Y^{4,*}_{j,\zeta} {}^2D^{a,i,b,j} {}^2T_{a,k,b,l} V_{k,i,l,j} \quad (8599)$$

Factorized expression

$$\tau^0_{\gamma,\alpha,w} = \sum_{a \in V} {}^2D^1_{a,w} W^1_{a,\alpha} Y^{1,*}_{a,\gamma} \quad (3r_D r_T r_V N_v) \quad (8600)$$

$$\tau^1_{\gamma,\alpha} = \sum_{a \in V} W^2_{a,\alpha} Y^1_{a,\gamma} \quad (2r_T r_V N_v) \quad (8601)$$

$$\tau^2_{\gamma,\alpha,i} = \sum_{\delta \in A} Y^2_{i,\delta} Z_{\delta,\gamma} \tau^1_{\delta,\alpha} \quad (3r_T^2 r_V N_o) \quad (8602)$$

$$\tau^3_{\gamma,\delta,\alpha,w} = \sum_{i \in O} {}^2D^2_{i,w} Y^{2,*}_{i,\delta} \tau^0_{\delta,\alpha,w} \tau^2_{\gamma,\alpha,i} \quad (4r_D r_T^2 r_V N_o) \quad (8603)$$

$$\tau^4_{\gamma,\alpha} = \sum_{a \in V} W^4_{a,\alpha} Y^3_{a,\gamma} \quad (2r_T r_V N_v) \quad (8604)$$

$$\tau^5_{\gamma,\alpha,a} = \sum_{\beta \in B} X_{\alpha,\beta} W^3_{a,\beta} \tau^4_{\gamma,\beta} \quad (3r_T r_V^2 N_v) \quad (8605)$$

$$\tau^6_{\gamma,\delta,w,a} = \sum_{\alpha \in B} \tau^5_{\gamma,\alpha,a} \tau^3_{\gamma,\delta,\alpha,w} \quad (2r_D r_T^2 r_V N_v) \quad (8606)$$

$$\tau^7_{\gamma,i,a} = \sum_{\delta \in A} \sum_{w \in D} {}^2D^3_{a,w} {}^2D^4_{i,w} Y^4_{i,\delta} \tau^6_{\delta,\gamma,w,a} \quad (4r_D r_T^2 N_o N_v) \quad (8607)$$

$${}^2R^3_{a,\gamma} \leftarrow \sum_{\delta \in A} \sum_{i \in O} \frac{1}{2} Z^*_{\delta,\gamma} Y^{4,*}_{i,\gamma} \tau^7_{\delta,i,a} \quad (3r_T^2 N_o N_v) \quad (8608)$$

Raw expression

$${}^2R^3_{b,\zeta} \leftarrow \sum_{\gamma \in A} \sum_{i \in O} \sum_{j \in O} \sum_{k \in O} \sum_{l \in O} \sum_{a \in V} \frac{1}{2} Y^{1,*}_{a,\gamma} Y^{2,*}_{i,\gamma} Z^*_{\gamma,\zeta} Y^{4,*}_{j,\zeta} {}^2D^{a,i,b,j} {}^2T_{b,k,a,l} V_{l,i,k,j} \quad (8609)$$

Factorized expression

$$\tau^0_{\gamma,\alpha,w} = \sum_{a \in V} {}^2D^1_{a,w} W^1_{a,\alpha} Y^{1,*}_{a,\gamma} \quad (3r_D r_T r_V N_v) \quad (8610)$$

$$\tau^1_{\gamma,\alpha} = \sum_{a \in V} W^2_{a,\alpha} Y^3_{a,\gamma} \quad (2r_T r_V N_v) \quad (8611)$$

$$\tau^2_{\gamma,\alpha,i} = \sum_{\delta \in A} Z_{\gamma,\delta} Y^4_{i,\delta} \tau^1_{\delta,\alpha} \quad (3r_T^2 r_V N_o) \quad (8612)$$

$$\tau^3_{\gamma,\delta,\alpha,w} = \sum_{i \in O} {}^2D^2_{i,w} Y^{2,*}_{i,\delta} \tau^0_{\delta,\alpha,w} \tau^2_{\gamma,\alpha,i} \quad (4r_D r_T^2 r_V N_o) \quad (8613)$$

$$\tau^4_{\gamma,\alpha} = \sum_{a \in V} W^4_{a,\alpha} Y^1_{a,\gamma} \quad (2r_T r_V N_v) \quad (8614)$$

$$\tau^5_{\gamma,\alpha,a} = \sum_{\beta \in B} X_{\alpha,\beta} W^3_{a,\beta} \tau^4_{\gamma,\beta} \quad (3r_T r_V^2 N_v) \quad (8615)$$

$$\tau^6_{\gamma,\delta,w,a} = \sum_{\alpha \in B} \tau^5_{\gamma,\alpha,a} \tau^3_{\gamma,\delta,\alpha,w} \quad (2r_D r_T^2 r_V N_v) \quad (8616)$$

$$\tau^7_{\gamma,i,a} = \sum_{\delta \in A} \sum_{w \in D} {}^2D^3_{a,w} {}^2D^4_{i,w} Y^2_{i,\delta} \tau^6_{\delta,\gamma,w,a} \quad (4r_D r_T^2 N_o N_v) \quad (8617)$$

$${}^2R^3_{a,\gamma} \leftarrow \sum_{\delta \in A} \sum_{i \in O} \frac{1}{2} Z^*_{\delta,\gamma} Y^{4,*}_{i,\gamma} \tau^7_{\delta,i,a} \quad (3r_T^2 N_o N_v) \quad (8618)$$

Raw expression

$${}^2R^3_{b,\zeta} \leftarrow - \sum_{\gamma \in A} \sum_{i \in O} \sum_{j \in O} \sum_{k \in O} \sum_{a \in V} \frac{1}{2} Y^{1,*}_{a,\gamma} Y^{2,*}_{i,\gamma} Z^*_{\gamma,\zeta} Y^{4,*}_{j,\zeta} f_{k,i} {}^2D^{a,i,b,j}_{a,k,b,j} \quad (8619)$$

Factorized expression

$$\tau^0_{\gamma,\delta,w} = \sum_{i \in O} {}^2D^4_{i,w} Y^4_{i,\gamma} Y^{4,*}_{i,\delta} \quad (3r_D r_T^2 N_o) \quad (8620)$$

$$\tau^1_{\gamma,\delta,w} = \sum_{a \in V} {}^2D^1_{a,w} Y^1_{a,\gamma} Y^{1,*}_{a,\delta} \quad (3r_D r_T^2 N_v) \quad (8621)$$

$$\tau^2_{\gamma,\delta,w} = \sum_{i \in O} {}^2D^2_{i,w} Y^2_{i,\gamma} Y^{2,*}_{i,\delta} \quad (3r_D r_T^2 N_o) \quad (8622)$$

$$\tau^3_{\gamma,\delta,w} = \sum_{\epsilon \in A} Z^*_{\epsilon,\delta} \tau^1_{\gamma,\epsilon,w} \tau^2_{\gamma,\epsilon,w} \quad (3r_D r_T^3) \quad (8623)$$

$$\tau^4_{\gamma,\delta,w} = \sum_{\epsilon \in A} Z_{\epsilon,\gamma} \tau^3_{\epsilon,\delta,w} \quad (2r_D r_T^3) \quad (8624)$$

$$\tau^5_{\gamma,a} = \sum_{b \in V} Y^3_{b,\gamma} f_{a,b} \quad (2r_T N_v^2) \quad (8625)$$

$${}^2R^3_{a,\gamma} \leftarrow \sum_{\delta \in A} \sum_{w \in D} \frac{1}{2} {}^2D^3_{a,w} \tau^5_{\delta,a} \tau^0_{\delta,\gamma,w} \tau^4_{\delta,\gamma,w} \quad (4r_D r_T^2 N_v) \quad (8626)$$

Raw expression

$${}^2R^3_{b,\zeta} \leftarrow - \sum_{\gamma \in A} \sum_{i \in O} \sum_{j \in O} \sum_{k \in O} \sum_{a \in V} \frac{1}{2} Y^{1,*}_{a,\gamma} Y^{2,*}_{i,\gamma} Z^*_{\gamma,\zeta} Y^{4,*}_{j,\zeta} f_{k,i} {}^2D^{a,i,b,j}_{a,b,j,k} \quad (8627)$$

Factorized expression

$$\tau^0_{\gamma,\delta,w} = \sum_{i \in O} {}^2D^4_{i,w} Y^2_{i,\gamma} Y^{4,*}_{i,\delta} \quad (3r_D r_T^2 N_o) \quad (8628)$$

$$\tau^1_{\gamma,\delta,w} = \sum_{i \in O} {}^2D^2_{i,w} Y^4_{i,\gamma} Y^{2,*}_{i,\delta} \quad (3r_D r_T^2 N_o) \quad (8629)$$

$$\tau^2_{\gamma,a} = \sum_{b \in V} Y^3_{b,\gamma} f_{a,b} \quad (2r_T N_v^2) \quad (8630)$$

$$\tau^3_{\gamma,\delta,w} = \sum_{a \in V} {}^2D^1_{a,w} Y^{1,*}_{a,\delta} \tau^2_{\gamma,a} \quad (3r_D r_T^2 N_v) \quad (8631)$$

$$\tau^4_{\gamma,\delta,w} = \sum_{\epsilon \in A} Z^*_{\epsilon,\delta} \tau^1_{\gamma,\epsilon,w} \tau^3_{\gamma,\epsilon,w} \quad (3r_D r_T^3) \quad (8632)$$

$$\tau^5_{\gamma,\delta,w} = \sum_{\epsilon \in A} Z_{\gamma,\epsilon} \tau^4_{\epsilon,\delta,w} \quad (2r_D r_T^3) \quad (8633)$$

$${}^2R^3_{a,\gamma} \leftarrow \sum_{\delta \in A} \sum_{w \in D} \frac{1}{2} {}^2D^3_{a,w} Y^1_{a,\delta} \tau^0_{\delta,\gamma,w} \tau^5_{\delta,\gamma,w} \quad (4r_D r_T^2 N_v) \quad (8634)$$

Raw expression

$${}^2R^3_{b,\zeta} \leftarrow - \sum_{\gamma \in A} \sum_{i \in O} \sum_{j \in O} \sum_{k \in O} \sum_{a \in V} \frac{1}{2} Y^{1,*}_{a,\gamma} Y^{2,*}_{i,\gamma} Z^*_{\gamma,\zeta} Y^{4,*}_{j,\zeta} f_{k,j} {}^2D^{a,i,b,j}_{a,i,b,k} \quad (8635)$$

Factorized expression

$$\tau^0_{\gamma,\delta,w} = \sum_{i \in O} {}^2D^4_{i,w} Y^4_{i,\gamma} Y^{4,*}_{i,\delta} \quad (3r_D r_T^2 N_o) \quad (8636)$$

$$\tau^1_{\gamma,\delta,w} = \sum_{i \in O} {}^2D^2_{i,w} Y^2_{i,\gamma} Y^{2,*}_{i,\delta} \quad (3r_D r_T^2 N_o) \quad (8637)$$

$$\tau^2_{\gamma,a} = \sum_{b \in V} Y^1_{b,\gamma} f_{a,b} \quad (2r_T N_v^2) \quad (8638)$$

$$\tau^3_{\gamma,\delta,w} = \sum_{a \in V} {}^2D^1_{a,w} Y^{1,*}_{a,\delta} \tau^2_{\gamma,a} \quad (3r_D r_T^2 N_v) \quad (8639)$$

$$\tau_{\gamma,\delta,w}^4 = \sum_{\epsilon \in A} Z_{\epsilon,\delta}^* \tau_{\gamma,\epsilon,w}^1 \tau_{\gamma,\epsilon,w}^3 \quad (3r_D r_T^3) \quad (8640)$$

$$\tau_{\gamma,\delta,w}^5 = \sum_{\epsilon \in A} Z_{\epsilon,\gamma} \tau_{\epsilon,\delta,w}^4 \quad (2r_D r_T^3) \quad (8641)$$

$${}^2R_{a,\gamma}^3 \leftarrow \sum_{\delta \in A} \sum_{w \in D} \frac{1}{2} {}^2D_{a,w}^3 Y_{a,\delta}^3 \tau_{\delta,\gamma,w}^0 \tau_{\delta,\gamma,w}^5 \quad (4r_D r_T^2 N_v) \quad (8642)$$

Raw expression

$${}^2R_{b,\zeta}^3 \leftarrow - \sum_{\gamma \in A} \sum_{i \in O} \sum_{j \in O} \sum_{k \in O} \sum_{a \in V} \frac{1}{2} Y_{a,\gamma}^{1,*} Y_{i,\gamma}^{2,*} Z_{\gamma,\zeta}^* Y_{j,\zeta}^{4,*} f_{k,j} {}^2D_{a,i,b,j} {}^2T_{b,k,a,i} \quad (8643)$$

Factorized expression

$$\tau_{\gamma,\delta,w}^0 = \sum_{i \in O} {}^2D_{i,w}^4 Y_{i,\gamma}^2 Y_{i,\delta}^{4,*} \quad (3r_D r_T^2 N_o) \quad (8644)$$

$$\tau_{\gamma,\delta,w}^1 = \sum_{a \in V} {}^2D_{a,w}^1 Y_{a,\gamma}^3 Y_{a,\delta}^{1,*} \quad (3r_D r_T^2 N_v) \quad (8645)$$

$$\tau_{\gamma,\delta,w}^2 = \sum_{i \in O} {}^2D_{i,w}^2 Y_{i,\gamma}^4 Y_{i,\delta}^{2,*} \quad (3r_D r_T^2 N_o) \quad (8646)$$

$$\tau_{\gamma,\delta,w}^3 = \sum_{\epsilon \in A} Z_{\epsilon,\delta}^* \tau_{\gamma,\epsilon,w}^1 \tau_{\gamma,\epsilon,w}^2 \quad (3r_D r_T^3) \quad (8647)$$

$$\tau_{\gamma,\delta,w}^4 = \sum_{\epsilon \in A} Z_{\gamma,\epsilon} \tau_{\epsilon,\delta,w}^3 \quad (2r_D r_T^3) \quad (8648)$$

$$\tau_{\gamma,a}^5 = \sum_{b \in V} Y_{b,\gamma}^1 f_{a,b} \quad (2r_T N_v^2) \quad (8649)$$

$${}^2R_{a,\gamma}^3 \leftarrow \sum_{\delta \in A} \sum_{w \in D} \frac{1}{2} {}^2D_{a,w}^3 \tau_{\delta,a}^5 \tau_{\delta,\gamma,w}^0 \tau_{\delta,\gamma,w}^4 \quad (4r_D r_T^2 N_v) \quad (8650)$$

### E. Contributions from $(H^1 T^1 T^1 T)_c$

Raw expression

$${}^2R_{b,\zeta}^3 \leftarrow - \sum_{\gamma \in A} \sum_{i \in O} \sum_{j \in O} \sum_{k \in O} \sum_{a \in V} \sum_{c \in V} \sum_{d \in V} {}^1T_{a,k} {}^1T_{c,i} {}^1T_{d,j} Y_{a,\gamma}^{1,*} Y_{i,\gamma}^{2,*} Z_{\gamma,\zeta}^* Y_{j,\zeta}^{4,*} {}^2D_{a,i,b,j} V_{b,d,k,c} \quad (8651)$$

Factorized expression

$$\tau_{\alpha,i}^0 = \sum_{a \in V} {}^1T_{a,i} W_{a,\alpha}^4 \quad (2r_V N_o N_v) \quad (8652)$$

$$\tau_{\gamma,\alpha,w}^1 = \sum_{i \in O} {}^2D_{i,w}^2 Y_{i,\gamma}^{2,*} \tau_{\alpha,i}^0 \quad (3r_D r_T r_V N_o) \quad (8653)$$

$$\tau_{\gamma,w,i}^2 = \sum_{a \in V} {}^2D_{a,w}^1 {}^1T_{a,i} Y_{a,\gamma}^{1,*} \quad (3r_D r_T N_o N_v) \quad (8654)$$

$$\tau_{\gamma,\alpha,w}^3 = \sum_{i \in O} W_{i,\alpha}^3 \tau_{\gamma,w,i}^2 \quad (2r_D r_T r_V N_o) \quad (8655)$$

$$\tau_{\gamma,\alpha,w}^4 = \sum_{\beta \in B} X_{\alpha,\beta} \tau_{\gamma,\beta,w}^1 \tau_{\gamma,\beta,w}^3 \quad (3r_D r_T r_V^2) \quad (8656)$$

$$\tau_{\gamma,\alpha,w}^5 = \sum_{\delta \in A} Z_{\delta,\gamma}^* \tau_{\delta,\alpha,w}^4 \quad (2r_D r_T^2 r_V) \quad (8657)$$

$$\tau_{\alpha,i}^6 = \sum_{a \in V} {}^1T_{a,i} W_{a,\alpha}^2 \quad (2r_V N_o N_v) \quad (8658)$$

$$\tau_{\gamma,\alpha,w}^7 = \sum_{i \in O} {}^2D_{i,w}^4 Y_{i,\gamma}^{4,*} \tau_{\alpha,i}^6 \quad (3r_D r_T r_V N_o) \quad (8659)$$

$$\tau_{\gamma,w,a}^8 = \sum_{\alpha \in B} W_{a,\alpha}^1 \tau_{\gamma,\alpha,w}^5 \tau_{\gamma,\alpha,w}^7 \quad (3r_D r_T r_V N_v) \quad (8660)$$

$${}^2R_{a,\gamma}^3 \leftarrow - \sum_{w \in D} {}^2D_{a,w}^3 \tau_{\gamma,w,a}^8 \quad (2r_D r_T N_v) \quad (8661)$$

Raw expression

$${}^2R_{b,\zeta}^3 \leftarrow - \sum_{\gamma \in A} \sum_{i \in O} \sum_{j \in O} \sum_{k \in O} \sum_{a \in V} \sum_{c \in V} \sum_{d \in V} {}^1T_{b,k} {}^1T_{c,i} {}^1T_{d,j} Y_{a,\gamma}^{1,*} Y_{i,\gamma}^{2,*} Z_{\gamma,\zeta}^* Y_{j,\zeta}^{4,*} {}^2D_{a,i,b,j} V_{a,c,k,d} \quad (8662)$$

Factorized expression

$$\tau_{\alpha,i}^0 = \sum_{a \in V} {}^1T_{a,i} W_{a,\alpha}^4 \quad (2r_V N_o N_v) \quad (8663)$$

$$\tau_{\gamma,\alpha,w}^1 = \sum_{i \in O} {}^2D_{i,w}^4 Y_{i,\gamma}^{4,*} \tau_{\alpha,i}^0 \quad (3r_D r_T r_V N_o) \quad (8664)$$

$$\tau^2_{\alpha,i} = \sum_{a \in V} {}^1T_{a,i} W^2_{a,\alpha} \quad (2r_V N_o N_v) \quad (8665)$$

$$\tau^4_{\gamma,\alpha,w} = \sum_{i \in O} W^1_{i,\alpha} \tau^3_{\gamma,w,i} \quad (2r_D r_T r_V N_o) \quad (8677)$$

$$\tau^3_{\gamma,\alpha,w} = \sum_{i \in O} {}^2D^2_{i,w} Y^{2,*}_{i,\gamma} \tau^2_{\alpha,i} \quad (3r_D r_T r_V N_o) \quad (8666)$$

$$\tau^5_{\gamma,\alpha,w} = \sum_{\beta \in B} X_{\beta,\alpha} \tau^2_{\gamma,\beta,w} \tau^4_{\gamma,\beta,w} \quad (3r_D r_T r_V^2) \quad (8678)$$

$$\tau^4_{\gamma,\alpha,w} = \sum_{a \in V} {}^2D^1_{a,w} W^1_{a,\alpha} Y^{1,*}_{a,\gamma} \quad (3r_D r_T r_V N_v) \quad (8667)$$

$$\tau^6_{\gamma,\alpha,w} = \sum_{\delta \in A} Z^*_{\delta,\gamma} \tau^5_{\delta,\alpha,w} \quad (2r_D r_T^2 r_V) \quad (8679)$$

$$\tau^5_{\gamma,\alpha,w} = \sum_{\beta \in B} X_{\beta,\alpha} \tau^3_{\gamma,\beta,w} \tau^4_{\gamma,\beta,w} \quad (3r_D r_T r_V^2) \quad (8668)$$

$$\tau^7_{\gamma,w,i} = \sum_{\alpha \in B} W^3_{i,\alpha} \tau^0_{\gamma,\alpha,w} \tau^6_{\gamma,\alpha,w} \quad (3r_D r_T r_V N_o) \quad (8680)$$

$$\tau^6_{\gamma,\alpha,w} = \sum_{\delta \in A} Z^*_{\delta,\gamma} \tau^5_{\delta,\alpha,w} \quad (2r_D r_T^2 r_V) \quad (8669)$$

$${}^2R^3_{a,\gamma} \leftarrow \sum_{w \in D} \sum_{i \in O} {}^2D^3_{a,w} {}^1T_{a,i} \tau^7_{\gamma,w,i} \quad (3r_D r_T N_o N_v) \quad (8681)$$

$$\tau^7_{\gamma,w,i} = \sum_{\alpha \in B} W^3_{i,\alpha} \tau^1_{\gamma,\alpha,w} \tau^6_{\gamma,\alpha,w} \quad (3r_D r_T r_V N_o) \quad (8670)$$

Raw expression

$${}^2R^3_{a,\gamma} \leftarrow - \sum_{w \in D} \sum_{i \in O} {}^2D^3_{a,w} {}^1T_{a,i} \tau^7_{\gamma,w,i} \quad (3r_D r_T N_o N_v) \quad (8671)$$

$${}^2R^3_{b,\zeta} \leftarrow \sum_{\gamma \in A} \sum_{i \in O} \sum_{j \in O} \sum_{k \in O} \sum_{l \in O} \sum_{a \in V} \sum_{c \in V} {}^1T_{a,l} {}^1T_{b,k} {}^1T_{c,j} Y^{1,*}_{a,\gamma} Y^{2,*}_{i,\gamma} Z^*_{\gamma,\zeta} Y^{4,*}_{j,\zeta} {}^2D^{a,i,b,j} V_{l,i,k,c} \quad (8682)$$

Factorized expression

$${}^2R^3_{b,\zeta} \leftarrow \sum_{\gamma \in A} \sum_{i \in O} \sum_{j \in O} \sum_{k \in O} \sum_{l \in O} \sum_{a \in V} \sum_{c \in V} {}^1T_{a,l} {}^1T_{b,k} {}^1T_{c,i} Y^{1,*}_{a,\gamma} Y^{2,*}_{i,\gamma} Z^*_{\gamma,\zeta} Y^{4,*}_{j,\zeta} {}^2D^{a,i,b,j} V_{l,c,k,j} \quad (8672)$$

$$\tau^0_{\alpha,i} = \sum_{a \in V} {}^1T_{a,i} W^4_{a,\alpha} \quad (2r_V N_o N_v) \quad (8683)$$

$$\tau^1_{\gamma,\alpha,w} = \sum_{i \in O} {}^2D^4_{i,w} Y^{4,*}_{i,\gamma} \tau^0_{\alpha,i} \quad (3r_D r_T r_V N_o) \quad (8684)$$

Factorized expression

$$\tau^0_{\gamma,\alpha,w} = \sum_{i \in O} {}^2D^4_{i,w} W^4_{i,\alpha} Y^{4,*}_{i,\gamma} \quad (3r_D r_T r_V N_o) \quad (8673)$$

$$\tau^2_{\gamma,w,i} = \sum_{a \in V} {}^2D^1_{a,w} {}^1T_{a,i} Y^{1,*}_{a,\gamma} \quad (3r_D r_T N_o N_v) \quad (8685)$$

$$\tau^1_{\alpha,i} = \sum_{a \in V} {}^1T_{a,i} W^2_{a,\alpha} \quad (2r_V N_o N_v) \quad (8674)$$

$$\tau^3_{\gamma,\alpha,w} = \sum_{i \in O} W^1_{i,\alpha} \tau^2_{\gamma,w,i} \quad (2r_D r_T r_V N_o) \quad (8686)$$

$$\tau^2_{\gamma,\alpha,w} = \sum_{i \in O} {}^2D^2_{i,w} Y^{2,*}_{i,\gamma} \tau^1_{\alpha,i} \quad (3r_D r_T r_V N_o) \quad (8675)$$

$$\tau^4_{\gamma,\alpha,w} = \sum_{i \in O} {}^2D^2_{i,w} W^2_{i,\alpha} Y^{2,*}_{i,\gamma} \quad (3r_D r_T r_V N_o) \quad (8687)$$

$$\tau^3_{\gamma,w,i} = \sum_{a \in V} {}^2D^1_{a,w} {}^1T_{a,i} Y^{1,*}_{a,\gamma} \quad (3r_D r_T N_o N_v) \quad (8676)$$

$$\tau^5_{\gamma,\alpha,w} = \sum_{\beta \in B} X_{\beta,\alpha} \tau^3_{\gamma,\beta,w} \tau^4_{\gamma,\beta,w} \quad (3r_D r_T r_V^2) \quad (8688)$$

$$\tau_{\gamma,\alpha,w}^6 = \sum_{\delta \in A} Z_{\delta,\gamma}^* \tau_{\delta,\alpha,w}^5 \quad (2r_D r_T^2 r_V) \quad (8689)$$

$$\tau_{\gamma,\delta,w}^8 = \sum_{\alpha \in B} \tau_{\gamma,\alpha}^7 \tau_{\delta,\alpha,w}^2 \tau_{\delta,\alpha,w}^3 \quad (3r_D r_T^2 r_V) \quad (8701)$$

$$\tau_{\gamma,w,i}^7 = \sum_{\alpha \in B} W_{i,\alpha}^3 \tau_{\gamma,\alpha,w}^1 \tau_{\gamma,\alpha,w}^6 \quad (3r_D r_T r_V N_o) \quad (8690)$$

$$\tau_{\gamma,\delta,w}^9 = \sum_{\epsilon \in A} Z_{\epsilon,\delta}^* \tau_{\gamma,\epsilon,w}^8 \quad (2r_D r_T^3) \quad (8702)$$

$${}^2R_{a,\gamma}^3 \leftarrow \sum_{w \in D} \sum_{i \in O} {}^2D_{a,w}^3 {}^1T_{a,i} \tau_{\gamma,w,i}^7 \quad (3r_D r_T N_o N_v) \quad (8691)$$

$${}^2R_{a,\gamma}^3 \leftarrow - \sum_{\delta \in A} \sum_{w \in D} {}^2D_{a,w}^3 Y_{a,\delta}^1 \tau_{\delta,\gamma,w}^0 \tau_{\delta,\gamma,w}^9 \quad (4r_D r_T^2 N_v) \quad (8703)$$

### F. Contributions from $(H^1 T^2 T)_c$

Raw expression

$${}^2R_{b,\zeta}^3 \leftarrow - \sum_{\gamma \in A} \sum_{i \in O} \sum_{j \in O} \sum_{k \in O} \sum_{a \in V} \sum_{c \in V} \frac{1}{2} {}^1T_{a,k} Y_{a,\gamma}^{1,*} Y_{i,\gamma}^{2,*} Z_{\gamma,\zeta}^* Y_{j,\zeta}^{4,*} f_{k,c} {}^2D_{a,i,b,j} {}^2T_{b,j,c,i} \quad (8692)$$

Factorized expression

$$\tau_{\gamma,\delta,w}^0 = \sum_{i \in O} {}^2D_{i,w}^4 Y_{i,\gamma}^2 Y_{i,\delta}^{4,*} \quad (3r_D r_T^2 N_o) \quad (8693)$$

$$\tau_{\gamma,w,i}^1 = \sum_{a \in V} {}^2D_{a,w}^1 {}^1T_{a,i} Y_{a,\gamma}^{1,*} \quad (3r_D r_T N_o N_v) \quad (8694)$$

$$\tau_{\gamma,\alpha,w}^2 = \sum_{i \in O} W_{i,\alpha}^1 \tau_{\gamma,w,i}^1 \quad (2r_D r_T r_V N_o) \quad (8695)$$

$$\tau_{\gamma,\alpha,w}^3 = \sum_{i \in O} {}^2D_{i,w}^2 W_{i,\alpha}^2 Y_{i,\gamma}^{2,*} \quad (3r_D r_T r_V N_o) \quad (8696)$$

$$\tau_{\gamma,\alpha}^4 = \sum_{a \in V} W_{a,\alpha}^4 Y_{a,\gamma}^3 \quad (2r_T r_V N_v) \quad (8697)$$

$$\tau_{\gamma,\alpha}^5 = \sum_{i \in O} W_{i,\alpha}^3 Y_{i,\gamma}^4 \quad (2r_T r_V N_o) \quad (8698)$$

$$\tau_{\gamma,\alpha}^6 = \sum_{\beta \in B} X_{\alpha,\beta} \tau_{\gamma,\beta}^4 \tau_{\gamma,\beta}^5 \quad (3r_T r_V^2) \quad (8699)$$

$$\tau_{\gamma,\alpha}^7 = \sum_{\delta \in A} Z_{\gamma,\delta} \tau_{\delta,\alpha}^6 \quad (2r_T^2 r_V) \quad (8700)$$

Raw expression

$${}^2R_{b,\zeta}^3 \leftarrow - \sum_{\gamma \in A} \sum_{i \in O} \sum_{j \in O} \sum_{k \in O} \sum_{a \in V} \sum_{c \in V} \frac{1}{2} {}^1T_{a,k} Y_{a,\gamma}^{1,*} Y_{i,\gamma}^{2,*} Z_{\gamma,\zeta}^* Y_{j,\zeta}^{4,*} f_{k,c} {}^2D_{a,i,b,j} {}^2T_{c,i,b,j} \quad (8704)$$

Factorized expression

$$\tau_{\gamma,\delta,w}^0 = \sum_{i \in O} {}^2D_{i,w}^4 Y_{i,\gamma}^4 Y_{i,\delta}^{4,*} \quad (3r_D r_T^2 N_o) \quad (8705)$$

$$\tau_{\gamma,w,i}^1 = \sum_{a \in V} {}^2D_{a,w}^1 {}^1T_{a,i} Y_{a,\gamma}^{1,*} \quad (3r_D r_T N_o N_v) \quad (8706)$$

$$\tau_{\gamma,\alpha,w}^2 = \sum_{i \in O} W_{i,\alpha}^1 \tau_{\gamma,w,i}^1 \quad (2r_D r_T r_V N_o) \quad (8707)$$

$$\tau_{\gamma,\alpha,w}^3 = \sum_{i \in O} {}^2D_{i,w}^2 W_{i,\alpha}^2 Y_{i,\gamma}^{2,*} \quad (3r_D r_T r_V N_o) \quad (8708)$$

$$\tau_{\gamma,\alpha}^4 = \sum_{a \in V} W_{a,\alpha}^4 Y_{a,\gamma}^1 \quad (2r_T r_V N_v) \quad (8709)$$

$$\tau_{\gamma,\alpha}^5 = \sum_{i \in O} W_{i,\alpha}^3 Y_{i,\gamma}^2 \quad (2r_T r_V N_o) \quad (8710)$$

$$\tau_{\gamma,\alpha}^6 = \sum_{\beta \in B} X_{\alpha,\beta} \tau_{\gamma,\beta}^4 \tau_{\gamma,\beta}^5 \quad (3r_T r_V^2) \quad (8711)$$

$$\tau_{\gamma,\alpha}^7 = \sum_{\delta \in A} Z_{\delta,\gamma} \tau_{\delta,\alpha}^6 \quad (2r_T^2 r_V) \quad (8712)$$

$$\tau_{\gamma,\delta,w}^8 = \sum_{\alpha \in B} \tau_{\gamma,\alpha}^7 \tau_{\delta,\alpha,w}^2 \tau_{\delta,\alpha,w}^3 \quad (3r_D r_T^2 r_V) \quad (8713)$$

$$\tau_{\gamma,\delta,w}^9 = \sum_{\epsilon \in A} Z_{\epsilon,\delta}^* \tau_{\gamma,\epsilon,w}^8 \quad (2r_D r_T^3) \quad (8714)$$

$${}^2R_{a,\gamma}^3 \leftarrow - \sum_{w \in D} \sum_{i \in O} {}^2D_{a,w}^3 {}^1T_{a,i} \tau_{\gamma,w,i}^9 \quad (3r_D r_T N_o N_v) \quad (8727)$$

$${}^2R_{a,\gamma}^3 \leftarrow - \sum_{\delta \in A} \sum_{w \in D} {}^2D_{a,w}^3 Y_{a,\delta}^3 \tau_{\delta,\gamma,w}^0 \tau_{\delta,\gamma,w}^9 \quad (4r_D r_T^2 N_v) \quad \text{Raw expression} \quad (8715)$$

Raw expression

$${}^2R_{b,\zeta}^3 \leftarrow - \sum_{\gamma \in A} \sum_{i \in O} \sum_{j \in O} \sum_{k \in O} \sum_{a \in V} \sum_{c \in V} \frac{1}{2} {}^1T_{b,k} Y_{a,\gamma}^{1,*} Y_{i,\gamma}^{2,*} Z_{\gamma,\zeta}^* Y_{j,\zeta}^{4,*} f_{k,c} {}^2D_{a,i,b,j} {}^2T_{c,j,a,i} \quad (8728)$$

Factorized expression

$${}^2R_{b,\zeta}^3 \leftarrow - \sum_{\gamma \in A} \sum_{i \in O} \sum_{j \in O} \sum_{k \in O} \sum_{a \in V} \sum_{c \in V} \frac{1}{2} {}^1T_{b,k} Y_{a,\gamma}^{1,*} Y_{i,\gamma}^{2,*} Z_{\gamma,\zeta}^* Y_{j,\zeta}^{4,*} f_{k,c} {}^2D_{a,i,b,j} {}^2T_{a,i,c,j} \quad (8716)$$

Factorized expression

$$\tau_{\gamma,\delta,w}^0 = \sum_{a \in V} {}^2D_{a,w}^1 Y_{a,\gamma}^3 Y_{a,\delta}^{1,*} \quad (3r_D r_T^2 N_v) \quad (8729)$$

$$\tau_{\gamma,\alpha}^0 = \sum_{a \in V} W_{a,\alpha}^2 Y_{a,\gamma}^3 \quad (2r_T r_V N_v) \quad (8717)$$

$$\tau_{\gamma,\delta,w}^1 = \sum_{i \in O} {}^2D_{i,w}^2 Y_{i,\gamma}^4 Y_{i,\delta}^{2,*} \quad (3r_D r_T^2 N_o) \quad (8730)$$

$$\tau_{\gamma,\alpha}^1 = \sum_{i \in O} W_{i,\alpha}^1 Y_{i,\gamma}^4 \quad (2r_T r_V N_o) \quad (8718)$$

$$\tau_{\gamma,\delta,w}^2 = \sum_{\epsilon \in A} Z_{\epsilon,\delta}^* \tau_{\gamma,\epsilon,w}^0 \tau_{\gamma,\epsilon,w}^1 \quad (3r_D r_T^3) \quad (8731)$$

$$\tau_{\gamma,\alpha}^2 = \sum_{\beta \in B} X_{\beta,\alpha} \tau_{\gamma,\beta}^0 \tau_{\gamma,\beta}^1 \quad (3r_T r_V^2) \quad (8719)$$

$$\tau_{\gamma,\alpha}^3 = \sum_{a \in V} W_{a,\alpha}^2 Y_{a,\gamma}^1 \quad (2r_T r_V N_v) \quad (8732)$$

$$\tau_{\gamma,\alpha}^3 = \sum_{\delta \in A} Z_{\gamma,\delta} \tau_{\delta,\alpha}^2 \quad (2r_T^2 r_V) \quad (8720)$$

$$\tau_{\gamma,\alpha}^4 = \sum_{i \in O} W_{i,\alpha}^1 Y_{i,\gamma}^2 \quad (2r_T r_V N_o) \quad (8733)$$

$$\tau_{\gamma,\delta,w}^4 = \sum_{a \in V} {}^2D_{a,w}^1 Y_{a,\gamma}^1 Y_{a,\delta}^{1,*} \quad (3r_D r_T^2 N_v) \quad (8721)$$

$$\tau_{\gamma,\alpha}^5 = \sum_{\beta \in B} X_{\beta,\alpha} \tau_{\gamma,\beta}^3 \tau_{\gamma,\beta}^4 \quad (3r_T r_V^2) \quad (8734)$$

$$\tau_{\gamma,\delta,w}^5 = \sum_{i \in O} {}^2D_{i,w}^2 Y_{i,\gamma}^2 Y_{i,\delta}^{2,*} \quad (3r_D r_T^2 N_o) \quad (8722)$$

$$\tau_{\gamma,\alpha}^6 = \sum_{\delta \in A} Z_{\delta,\gamma} \tau_{\delta,\alpha}^5 \quad (2r_T^2 r_V) \quad (8735)$$

$$\tau_{\gamma,\delta,w}^6 = \sum_{\epsilon \in A} Z_{\epsilon,\delta}^* \tau_{\gamma,\epsilon,w}^4 \tau_{\gamma,\epsilon,w}^5 \quad (3r_D r_T^3) \quad (8723)$$

$$\tau_{\gamma,\alpha,w}^7 = \sum_{\delta \in A} \tau_{\delta,\alpha}^6 \tau_{\delta,\gamma,w}^2 \quad (2r_D r_T^2 r_V) \quad (8736)$$

$$\tau_{\gamma,\alpha,w}^7 = \sum_{\delta \in A} \tau_{\delta,\alpha}^3 \tau_{\delta,\gamma,w}^6 \quad (2r_D r_T^2 r_V) \quad (8724)$$

$$\tau_{\gamma,\alpha,w}^8 = \sum_{i \in O} {}^2D_{i,w}^4 W_{i,\alpha}^4 Y_{i,\gamma}^{4,*} \quad (3r_D r_T r_V N_o) \quad (8737)$$

$$\tau_{\gamma,\alpha,w}^8 = \sum_{i \in O} {}^2D_{i,w}^4 W_{i,\alpha}^4 Y_{i,\gamma}^{4,*} \quad (3r_D r_T r_V N_o) \quad (8725)$$

$$\tau_{\gamma,w,i}^9 = \sum_{\alpha \in B} W_{i,\alpha}^3 \tau_{\gamma,\alpha,w}^7 \tau_{\gamma,\alpha,w}^8 \quad (3r_D r_T r_V N_o) \quad (8738)$$

$$\tau_{\gamma,w,i}^9 = \sum_{\alpha \in B} W_{i,\alpha}^3 \tau_{\gamma,\alpha,w}^7 \tau_{\gamma,\alpha,w}^8 \quad (3r_D r_T r_V N_o) \quad (8726)$$

$${}^2R_{a,\gamma}^3 \leftarrow - \sum_{w \in D} \sum_{i \in O} {}^2D_{a,w}^3 {}^1T_{a,i} \tau_{\gamma,w,i}^9 \quad (3r_D r_T N_o N_v) \quad (8739)$$

Raw expression

$${}^2R^3_{b,\zeta} \leftarrow - \sum_{\gamma \in A} \sum_{i \in O} \sum_{j \in O} \sum_{k \in O} \sum_{a \in V} \sum_{c \in V} \frac{1}{2} {}^1T_{c,i} {}^{Y^{1,*}}_{a,\gamma} {}^{Y^{2,*}}_{i,\gamma} {}^{Z^*}_{\gamma,\zeta} {}^{Y^{4,*}}_{j,\zeta} f_{k,c} {}^2D^{a,i,b,j} {}^2T_{a,k,b,j} \quad (8740)$$

Factorized expression

$$\tau^0_{\alpha,i} = \sum_{a \in V} {}^1T_{a,i} W^2_{a,\alpha} \quad (2r_V N_o N_v) \quad (8741)$$

$$\tau^1_{\alpha} = \sum_{i \in O} W^1_{i,\alpha} \tau^0_{\alpha,i} \quad (2r_V N_o) \quad (8742)$$

$$\tau^2_{\alpha} = \sum_{\beta \in B} \tau^1_{\beta} X_{\beta,\alpha} \quad (2r_V^2) \quad (8743)$$

$$\tau^3_{i,j} = \sum_{\alpha \in B} \tau^2_{\alpha} W^3_{i,\alpha} W^4_{j,\alpha} \quad (3r_V N_o^2) \quad (8744)$$

$$\tau^4_{\gamma,i} = \sum_{j \in O} Y^4_{j,\gamma} \tau^3_{j,i} \quad (2r_T N_o^2) \quad (8745)$$

$$\tau^5_{\gamma,\delta,w} = \sum_{i \in O} {}^2D^4_{i,w} Y^{4,*}_{i,\delta} \tau^4_{\gamma,i} \quad (3r_D r_T^2 N_o) \quad (8746)$$

$$\tau^6_{\gamma,\delta,w} = \sum_{a \in V} {}^2D^1_{a,w} Y^1_{a,\gamma} Y^{1,*}_{a,\delta} \quad (3r_D r_T^2 N_v) \quad (8747)$$

$$\tau^7_{\gamma,\delta,w} = \sum_{i \in O} {}^2D^2_{i,w} Y^2_{i,\gamma} Y^{2,*}_{i,\delta} \quad (3r_D r_T^2 N_o) \quad (8748)$$

$$\tau^8_{\gamma,\delta,w} = \sum_{\epsilon \in A} Z^*_{\epsilon,\delta} \tau^6_{\gamma,\epsilon,w} \tau^7_{\gamma,\epsilon,w} \quad (3r_D r_T^3) \quad (8749)$$

$$\tau^9_{\gamma,\delta,w} = \sum_{\epsilon \in A} Z_{\epsilon,\gamma} \tau^8_{\epsilon,\delta,w} \quad (2r_D r_T^3) \quad (8750)$$

$${}^2R^3_{a,\gamma} \leftarrow - \sum_{\delta \in A} \sum_{w \in D} {}^2D^3_{a,w} Y^3_{a,\delta} \tau^5_{\delta,\gamma,w} \tau^9_{\delta,\gamma,w} \quad (4r_D r_T^2 N_v) \quad (8751)$$

Raw expression

$${}^2R^3_{b,\zeta} \leftarrow - \sum_{\gamma \in A} \sum_{i \in O} \sum_{j \in O} \sum_{k \in O} \sum_{a \in V} \sum_{c \in V} \frac{1}{2} {}^1T_{c,i} {}^{Y^{1,*}}_{a,\gamma} {}^{Y^{2,*}}_{i,\gamma} {}^{Z^*}_{\gamma,\zeta} {}^{Y^{4,*}}_{j,\zeta} f_{k,c} {}^2D^{a,i,b,j} {}^2T_{b,j,a,k} \quad (8752)$$

Factorized expression

$$\tau^0_{\alpha,i} = \sum_{a \in V} {}^1T_{a,i} W^2_{a,\alpha} \quad (2r_V N_o N_v) \quad (8753)$$

$$\tau^1_{\alpha} = \sum_{i \in O} W^1_{i,\alpha} \tau^0_{\alpha,i} \quad (2r_V N_o) \quad (8754)$$

$$\tau^2_{\alpha} = \sum_{\beta \in B} \tau^1_{\beta} X_{\beta,\alpha} \quad (2r_V^2) \quad (8755)$$

$$\tau^3_{i,j} = \sum_{\alpha \in B} \tau^2_{\alpha} W^3_{i,\alpha} W^4_{j,\alpha} \quad (3r_V N_o^2) \quad (8756)$$

$$\tau^4_{\gamma,i} = \sum_{j \in O} Y^2_{j,\gamma} \tau^3_{j,i} \quad (2r_T N_o^2) \quad (8757)$$

$$\tau^5_{\gamma,\delta,w} = \sum_{i \in O} {}^2D^4_{i,w} Y^{4,*}_{i,\delta} \tau^4_{\gamma,i} \quad (3r_D r_T^2 N_o) \quad (8758)$$

$$\tau^6_{\gamma,\delta,w} = \sum_{a \in V} {}^2D^1_{a,w} Y^3_{a,\gamma} Y^{1,*}_{a,\delta} \quad (3r_D r_T^2 N_v) \quad (8759)$$

$$\tau^7_{\gamma,\delta,w} = \sum_{i \in O} {}^2D^2_{i,w} Y^4_{i,\gamma} Y^{2,*}_{i,\delta} \quad (3r_D r_T^2 N_o) \quad (8760)$$

$$\tau^8_{\gamma,\delta,w} = \sum_{\epsilon \in A} Z^*_{\epsilon,\delta} \tau^6_{\gamma,\epsilon,w} \tau^7_{\gamma,\epsilon,w} \quad (3r_D r_T^3) \quad (8761)$$

$$\tau^9_{\gamma,\delta,w} = \sum_{\epsilon \in A} Z_{\gamma,\epsilon} \tau^8_{\epsilon,\delta,w} \quad (2r_D r_T^3) \quad (8762)$$

$${}^2R^3_{a,\gamma} \leftarrow - \sum_{\delta \in A} \sum_{w \in D} {}^2D^3_{a,w} Y^1_{a,\delta} \tau^5_{\delta,\gamma,w} \tau^9_{\delta,\gamma,w} \quad (4r_D r_T^2 N_v) \quad (8763)$$

Raw expression

$${}^2R^3_{b,\zeta} \leftarrow - \sum_{\gamma \in A} \sum_{i \in O} \sum_{j \in O} \sum_{k \in O} \sum_{a \in V} \sum_{c \in V} \frac{1}{2} {}^1T_{c,j} {}^{Y^{1,*}}_{a,\gamma} {}^{Y^{2,*}}_{i,\gamma} {}^{Z^*}_{\gamma,\zeta} {}^{Y^{4,*}}_{j,\zeta} f_{k,c} {}^2D^{a,i,b,j} {}^2T_{a,i,b,k} \quad (8764)$$

Factorized expression

$$\tau^0_{\gamma,\delta,w} = \sum_{i \in O} {}^2D^4_{i,w} Y^4_{i,\gamma} Y^{4,*}_{i,\delta} \quad (3r_D r_T^2 N_o) \quad (8765)$$



$$\tau^1_{\gamma,\delta,w} = \sum_{a \in V} {}^2D^1_{a,w} Y^1_{a,\gamma} Y^{1,*}_{a,\delta} \quad (3r_D r_T^2 N_v) \quad (8766)$$

$$\tau^2_{\alpha,i} = \sum_{a \in V} {}^1T_{a,i} W^4_{a,\alpha} \quad (2r_V N_o N_v) \quad (8779)$$

$$\tau^2_{\alpha,i} = \sum_{a \in V} {}^1T_{a,i} W^4_{a,\alpha} \quad (2r_V N_o N_v) \quad (8767)$$

$$\tau^3_{\alpha} = \sum_{i \in O} W^3_{i,\alpha} \tau^2_{\alpha,i} \quad (2r_V N_o) \quad (8780)$$

$$\tau^3_{\alpha} = \sum_{i \in O} W^3_{i,\alpha} \tau^2_{\alpha,i} \quad (2r_V N_o) \quad (8768)$$

$$\tau^4_{\alpha} = \sum_{\beta \in B} \tau^3_{\beta} X_{\alpha,\beta} \quad (2r_V^2) \quad (8781)$$

$$\tau^4_{\alpha} = \sum_{\beta \in B} \tau^3_{\beta} X_{\alpha,\beta} \quad (2r_V^2) \quad (8769)$$

$$\tau^5_{i,j} = \sum_{\alpha \in B} \tau^4_{\alpha} W^1_{i,\alpha} W^2_{j,\alpha} \quad (3r_V N_o^2) \quad (8782)$$

$$\tau^5_{i,j} = \sum_{\alpha \in B} \tau^4_{\alpha} W^1_{i,\alpha} W^2_{j,\alpha} \quad (3r_V N_o^2) \quad (8770)$$

$$\tau^6_{\gamma,i} = \sum_{j \in O} Y^4_{j,\gamma} \tau^5_{j,i} \quad (2r_T N_o^2) \quad (8783)$$

$$\tau^6_{\gamma,i} = \sum_{j \in O} Y^2_{j,\gamma} \tau^5_{j,i} \quad (2r_T N_o^2) \quad (8771)$$

$$\tau^7_{\gamma,\delta,w} = \sum_{i \in O} {}^2D^2_{i,w} Y^{2,*}_{i,\delta} \tau^6_{\gamma,i} \quad (3r_D r_T^2 N_o) \quad (8784)$$

$$\tau^7_{\gamma,\delta,w} = \sum_{i \in O} {}^2D^2_{i,w} Y^{2,*}_{i,\delta} \tau^6_{\gamma,i} \quad (3r_D r_T^2 N_o) \quad (8772)$$

$$\tau^8_{\gamma,\delta,w} = \sum_{\epsilon \in A} Z^*_{\epsilon,\delta} \tau^1_{\gamma,\epsilon,w} \tau^7_{\gamma,\epsilon,w} \quad (3r_D r_T^3) \quad (8785)$$

$$\tau^8_{\gamma,\delta,w} = \sum_{\epsilon \in A} Z^*_{\epsilon,\delta} \tau^1_{\gamma,\epsilon,w} \tau^7_{\gamma,\epsilon,w} \quad (3r_D r_T^3) \quad (8773)$$

$$\tau^9_{\gamma,\delta,w} = \sum_{\epsilon \in A} Z_{\gamma,\epsilon} \tau^8_{\epsilon,\delta,w} \quad (2r_D r_T^3) \quad (8786)$$

$$\tau^9_{\gamma,\delta,w} = \sum_{\epsilon \in A} Z_{\epsilon,\gamma} \tau^8_{\epsilon,\delta,w} \quad (2r_D r_T^3) \quad (8774)$$

$${}^2R^3_{a,\gamma} \leftarrow - \sum_{\delta \in A} \sum_{w \in D} {}^2D^3_{a,w} Y^1_{a,\delta} \tau^0_{\delta,\gamma,w} \tau^9_{\delta,\gamma,w} \quad (4r_D r_T^2 N_v) \quad (8787)$$

Raw expression

$${}^2R^3_{a,\gamma} \leftarrow - \sum_{\delta \in A} \sum_{w \in D} {}^2D^3_{a,w} Y^3_{a,\delta} \tau^0_{\delta,\gamma,w} \tau^9_{\delta,\gamma,w} \quad (4r_D r_T^2 N_v) \quad (8775)$$

$${}^2R^3_{b,\zeta} \leftarrow \sum_{\gamma \in A} \sum_{i \in O} \sum_{j \in O} \sum_{k \in O} \sum_{l \in O} \sum_{a \in V} \sum_{c \in V} \frac{1}{2} {}^1T_{a,k} Y^{1,*}_{a,\gamma} Y^{2,*}_{i,\gamma} Z^*_{\gamma,\zeta} Y^{4,*}_{j,\zeta} {}^2D^{a,i,b,j} {}^2T_{b,j,c,l} V_{l,i,k,c} \quad (8788)$$

Raw expression

Factorized expression

$${}^2R^3_{b,\zeta} \leftarrow - \sum_{\gamma \in A} \sum_{i \in O} \sum_{j \in O} \sum_{k \in O} \sum_{a \in V} \sum_{c \in V} \frac{1}{2} {}^1T_{c,j} Y^{1,*}_{a,\gamma} Y^{2,*}_{i,\gamma} Z^*_{\gamma,\zeta} Y^{4,*}_{j,\zeta} f_{k,c} {}^2D^{a,i,b,j} {}^2T_{b,k,a,i} \quad (8776)$$

$$\tau^0_{\gamma,w,i} = \sum_{a \in V} {}^2D^1_{a,w} {}^1T_{a,i} Y^{1,*}_{a,\gamma} \quad (3r_D r_T N_o N_v) \quad (8789)$$

Factorized expression

$$\tau^0_{\gamma,\delta,w} = \sum_{i \in O} {}^2D^4_{i,w} Y^2_{i,\gamma} Y^{4,*}_{i,\delta} \quad (3r_D r_T^2 N_o) \quad (8777)$$

$$\tau^1_{\gamma,w,i,j} = \sum_{\delta \in A} {}^2D^2_{i,w} Y^{2,*}_{i,\delta} Z^*_{\delta,\gamma} \tau^0_{\delta,w,j} \quad (4r_D r_T^2 N_o^2) \quad (8790)$$

$$\tau^1_{\gamma,\delta,w} = \sum_{a \in V} {}^2D^1_{a,w} Y^3_{a,\gamma} Y^{1,*}_{a,\delta} \quad (3r_D r_T^2 N_v) \quad (8778)$$

$$\tau^2_{\gamma,\alpha,w,i} = \sum_{j \in O} W^1_{j,\alpha} \tau^1_{\gamma,w,i,j} \quad (2r_D r_T r_V N_o^2) \quad (8791)$$

$$\tau^3_{\gamma,\alpha} = \sum_{a \in V} W^2_{a,\alpha} Y^3_{a,\gamma} \quad (2r_T r_V N_v) \quad (8792)$$

$$\tau^4_{\gamma,\alpha,i} = \sum_{\delta \in A} Z_{\gamma,\delta} Y^4_{i,\delta} \tau^3_{\delta,\alpha} \quad (3r_T^2 r_V N_o) \quad (8793)$$

$$\tau^5_{\gamma,\delta,\alpha,w} = \sum_{i \in O} \tau^4_{\gamma,\alpha,i} \tau^2_{\delta,\alpha,w,i} \quad (2r_D r_T^2 r_V N_o) \quad (8794)$$

$$\tau^6_{\alpha,i,j} = \sum_{\beta \in B} X_{\alpha,\beta} W^3_{i,\beta} W^4_{j,\beta} \quad (3r_V^2 N_o^2) \quad (8795)$$

$$\tau^7_{\gamma,\alpha,i} = \sum_{j \in O} Y^2_{j,\gamma} \tau^6_{\alpha,j,i} \quad (2r_T r_V N_o^2) \quad (8796)$$

$$\tau^8_{\gamma,\delta,w,i} = \sum_{\alpha \in B} \tau^7_{\gamma,\alpha,i} \tau^5_{\gamma,\delta,\alpha,w} \quad (2r_D r_T^2 r_V N_o) \quad (8797)$$

$$\tau^9_{\gamma,\delta,w} = \sum_{i \in O} {}^2D^4_{i,w} Y^{4,*}_{i,\delta} \tau^8_{\gamma,\delta,w,i} \quad (3r_D r_T^2 N_o) \quad (8798)$$

$${}^2R^3_{a,\gamma} \leftarrow \sum_{\delta \in A} \sum_{w \in D} \frac{1}{2} {}^2D^3_{a,w} Y^1_{a,\delta} \tau^9_{\delta,\gamma,w} \quad (3r_D r_T^2 N_v) \quad (8799)$$

Raw expression

$${}^2R^3_{b,\zeta} \leftarrow \sum_{\gamma \in A} \sum_{i \in O} \sum_{j \in O} \sum_{k \in O} \sum_{l \in O} \sum_{a \in V} \sum_{c \in V} \frac{1}{2} {}^1T_{a,k} Y^{1,*}_{a,\gamma} Y^{2,*}_{i,\gamma} Z^*_{\gamma,\zeta} Y^{4,*}_{j,\zeta} {}^2D^{a,i,b,j} {}^2T_{b,l,c,i} V_{k,c,l,j} \quad (8800)$$

Factorized expression

$$\tau^0_{\gamma,w,i} = \sum_{a \in V} {}^2D^1_{a,w} {}^1T_{a,i} Y^{1,*}_{a,\gamma} \quad (3r_D r_T N_o N_v) \quad (8801)$$

$$\tau^1_{\gamma,w,i,j} = \sum_{\delta \in A} {}^2D^2_{i,w} Y^{2,*}_{i,\delta} Z^*_{\delta,\gamma} \tau^0_{\delta,w,j} \quad (4r_D r_T^2 N_o^2) \quad (8802)$$

$$\tau^2_{\gamma,\alpha,w,i} = \sum_{j \in O} W^1_{j,\alpha} \tau^1_{\gamma,w,i,j} \quad (2r_D r_T r_V N_o^2) \quad (8803)$$

$$\tau^3_{\gamma,\alpha} = \sum_{a \in V} W^2_{a,\alpha} Y^1_{a,\gamma} \quad (2r_T r_V N_v) \quad (8804)$$

$$\tau^4_{\gamma,\alpha,i} = \sum_{\delta \in A} Y^2_{i,\delta} Z_{\delta,\gamma} \tau^3_{\delta,\alpha} \quad (3r_T^2 r_V N_o) \quad (8805)$$

$$\tau^5_{\gamma,\delta,\alpha,w} = \sum_{i \in O} \tau^4_{\gamma,\alpha,i} \tau^2_{\delta,\alpha,w,i} \quad (2r_D r_T^2 r_V N_o) \quad (8806)$$

$$\tau^6_{\alpha,i,j} = \sum_{\beta \in B} X_{\alpha,\beta} W^3_{i,\beta} W^4_{j,\beta} \quad (3r_V^2 N_o^2) \quad (8807)$$

$$\tau^7_{\gamma,\alpha,i} = \sum_{j \in O} Y^4_{j,\gamma} \tau^6_{\alpha,j,i} \quad (2r_T r_V N_o^2) \quad (8808)$$

$$\tau^8_{\gamma,\delta,w,i} = \sum_{\alpha \in B} \tau^7_{\gamma,\alpha,i} \tau^5_{\gamma,\delta,\alpha,w} \quad (2r_D r_T^2 r_V N_o) \quad (8809)$$

$$\tau^9_{\gamma,\delta,w} = \sum_{i \in O} {}^2D^4_{i,w} Y^{4,*}_{i,\delta} \tau^8_{\gamma,\delta,w,i} \quad (3r_D r_T^2 N_o) \quad (8810)$$

$${}^2R^3_{a,\gamma} \leftarrow \sum_{\delta \in A} \sum_{w \in D} \frac{1}{2} {}^2D^3_{a,w} Y^3_{a,\delta} \tau^9_{\delta,\gamma,w} \quad (3r_D r_T^2 N_v) \quad (8811)$$

Raw expression

$${}^2R^3_{b,\zeta} \leftarrow \sum_{\gamma \in A} \sum_{i \in O} \sum_{j \in O} \sum_{k \in O} \sum_{l \in O} \sum_{a \in V} \sum_{c \in V} \frac{1}{2} {}^1T_{a,k} Y^{1,*}_{a,\gamma} Y^{2,*}_{i,\gamma} Z^*_{\gamma,\zeta} Y^{4,*}_{j,\zeta} {}^2D^{a,i,b,j} {}^2T_{b,l,c,j} V_{k,i,l,c} \quad (8812)$$

Factorized expression

$$\tau^0_{\gamma,\alpha} = \sum_{i \in O} W^3_{i,\alpha} Y^2_{i,\gamma} \quad (2r_T r_V N_o) \quad (8813)$$

$$\tau^1_{\gamma,\alpha} = \sum_{a \in V} W^4_{a,\alpha} Y^3_{a,\gamma} \quad (2r_T r_V N_v) \quad (8814)$$

$$\tau^2_{\gamma,\alpha,i} = \sum_{\delta \in A} Z_{\gamma,\delta} Y^4_{i,\delta} \tau^1_{\delta,\alpha} \quad (3r_T^2 r_V N_o) \quad (8815)$$

$$\tau^3_{\gamma,w,i} = \sum_{a \in V} {}^2D^1_{a,w} {}^1T_{a,i} Y^{1,*}_{a,\gamma} \quad (3r_D r_T N_o N_v) \quad (8816)$$

$$\tau^4_{\gamma,\alpha,w} = \sum_{i \in O} W^1_{i,\alpha} \tau^3_{\gamma,w,i} \quad (2r_D r_T r_V N_o) \quad (8817)$$

$$\tau^4_{\gamma,\alpha,w} = \sum_{i \in O} W^1_{i,\alpha} \tau^3_{\gamma,w,i} \quad (2r_D r_T r_V N_o) \quad (8829)$$

$$\tau^5_{\gamma,\alpha,w} = \sum_{i \in O} {}^2D^2_{i,w} W^2_{i,\alpha} Y^{2,*}_{i,\gamma} \quad (3r_D r_T r_V N_o) \quad (8818)$$

$$\tau^5_{\gamma,\alpha,w} = \sum_{i \in O} {}^2D^2_{i,w} W^2_{i,\alpha} Y^{2,*}_{i,\gamma} \quad (3r_D r_T r_V N_o) \quad (8830)$$

$$\tau^6_{\gamma,\alpha,w} = \sum_{\beta \in B} X_{\beta,\alpha} \tau^4_{\gamma,\beta,w} \tau^5_{\gamma,\beta,w} \quad (3r_D r_T r_V^2) \quad (8819)$$

$$\tau^6_{\gamma,\alpha,w} = \sum_{\beta \in B} X_{\beta,\alpha} \tau^4_{\gamma,\beta,w} \tau^5_{\gamma,\beta,w} \quad (3r_D r_T r_V^2) \quad (8831)$$

$$\tau^7_{\gamma,\alpha,w} = \sum_{\delta \in A} Z^*_{\delta,\gamma} \tau^6_{\delta,\alpha,w} \quad (2r_D r_T^2 r_V) \quad (8820)$$

$$\tau^7_{\gamma,\alpha,w} = \sum_{\delta \in A} Z^*_{\delta,\gamma} \tau^6_{\delta,\alpha,w} \quad (2r_D r_T^2 r_V) \quad (8832)$$

$$\tau^8_{\gamma,\delta,w,i} = \sum_{\alpha \in B} \tau^0_{\gamma,\alpha} \tau^2_{\gamma,\alpha,i} \tau^7_{\delta,\alpha,w} \quad (3r_D r_T^2 r_V N_o) \quad (8821)$$

$$\tau^8_{\gamma,\delta,w,i} = \sum_{\alpha \in B} \tau^2_{\gamma,\alpha} \tau^1_{\gamma,\alpha,i} \tau^7_{\delta,\alpha,w} \quad (3r_D r_T^2 r_V N_o) \quad (8833)$$

$$\tau^9_{\gamma,\delta,w} = \sum_{i \in O} {}^2D^4_{i,w} Y^{4,*}_{i,\delta} \tau^8_{\gamma,\delta,w,i} \quad (3r_D r_T^2 N_o) \quad (8822)$$

$$\tau^9_{\gamma,\delta,w} = \sum_{i \in O} {}^2D^4_{i,w} Y^{4,*}_{i,\delta} \tau^8_{\gamma,\delta,w,i} \quad (3r_D r_T^2 N_o) \quad (8834)$$

$${}^2R^3_{a,\gamma} \leftarrow \sum_{\delta \in A} \sum_{w \in D} \frac{1}{2} {}^2D^3_{a,w} Y^1_{a,\delta} \tau^9_{\delta,\gamma,w} \quad (3r_D r_T^2 N_v) \quad (8823)$$

$${}^2R^3_{a,\gamma} \leftarrow \sum_{\delta \in A} \sum_{w \in D} \frac{1}{2} {}^2D^3_{a,w} Y^3_{a,\delta} \tau^9_{\delta,\gamma,w} \quad (3r_D r_T^2 N_v) \quad (8835)$$

Raw expression

$${}^2R^3_{b,\zeta} \leftarrow \sum_{\gamma \in A} \sum_{i \in O} \sum_{j \in O} \sum_{k \in O} \sum_{l \in O} \sum_{a \in V} \sum_{c \in V} \frac{1}{2} {}^1T_{a,k} Y^{1,*}_{a,\gamma} Y^{2,*}_{i,\gamma} Z^*_{\gamma,\zeta} Y^{4,*}_{j,\zeta} {}^2D^{a,i,b,j} {}^2T_{c,i,b,l} V_{k,c,l,j} \quad (8824)$$

Raw expression

$${}^2R^3_{b,\zeta} \leftarrow \sum_{\gamma \in A} \sum_{i \in O} \sum_{j \in O} \sum_{k \in O} \sum_{l \in O} \sum_{a \in V} \sum_{c \in V} \frac{1}{2} {}^1T_{a,k} Y^{1,*}_{a,\gamma} Y^{2,*}_{i,\gamma} Z^*_{\gamma,\zeta} Y^{4,*}_{j,\zeta} {}^2D^{a,i,b,j} {}^2T_{c,j,b,l} V_{k,i,l,c} \quad (8836)$$

Factorized expression

$$\tau^0_{\gamma,\alpha} = \sum_{a \in V} W^4_{a,\alpha} Y^1_{a,\gamma} \quad (2r_T r_V N_v) \quad (8825)$$

$$\tau^0_{\gamma,\delta,w} = \sum_{i \in O} {}^2D^4_{i,w} Y^2_{i,\gamma} Y^{4,*}_{i,\delta} \quad (3r_D r_T^2 N_o) \quad (8837)$$

$$\tau^1_{\gamma,\alpha,i} = \sum_{\delta \in A} Y^2_{i,\delta} Z_{\delta,\gamma} \tau^0_{\delta,\alpha} \quad (3r_T^2 r_V N_o) \quad (8826)$$

$$\tau^1_{\gamma,w,i} = \sum_{a \in V} {}^2D^1_{a,w} {}^1T_{a,i} Y^{1,*}_{a,\gamma} \quad (3r_D r_T N_o N_v) \quad (8838)$$

$$\tau^2_{\gamma,\alpha} = \sum_{i \in O} W^3_{i,\alpha} Y^4_{i,\gamma} \quad (2r_T r_V N_o) \quad (8827)$$

$$\tau^2_{\alpha,i,j} = \sum_{\beta \in B} W^1_{i,\beta} W^2_{j,\beta} X_{\beta,\alpha} \quad (3r_V^2 N_o^2) \quad (8839)$$

$$\tau^3_{\gamma,w,i} = \sum_{a \in V} {}^2D^1_{a,w} {}^1T_{a,i} Y^{1,*}_{a,\gamma} \quad (3r_D r_T N_o N_v) \quad (8828)$$

$$\tau^3_{\gamma,\alpha,i} = \sum_{j \in O} Y^4_{j,\gamma} \tau^2_{\alpha,j,i} \quad (2r_T r_V N_o^2) \quad (8840)$$

$$\tau^4_{\gamma,\alpha} = \sum_{a \in V} W^4_{a,\alpha} Y^3_{a,\gamma} \quad (2r_T r_V N_v) \quad (8841)$$

$$\tau^6_{\gamma,i,j} = \sum_{\delta \in A} Z_{\delta,\gamma} \tau^5_{\delta,i,j} \quad (2r_T^2 N_o^2) \quad (8854)$$

$$\tau^5_{\gamma,i,j} = \sum_{\alpha \in B} W^3_{j,\alpha} \tau^4_{\gamma,\alpha} \tau^3_{\gamma,\alpha,i} \quad (3r_T r_V N_o^2) \quad (8842)$$

$$\tau^7_{\gamma,\delta,w} = \sum_{i \in O} \sum_{j \in O} {}^2D^2_{i,w} Y^{2,*}_{i,\delta} \tau^1_{\delta,w,j} \tau^6_{\gamma,i,j} \quad (4r_D r_T^2 N_o^2) \quad (8855)$$

$$\tau^6_{\gamma,i,j} = \sum_{\delta \in A} Z_{\gamma,\delta} \tau^5_{\delta,i,j} \quad (2r_T^2 N_o^2) \quad (8843)$$

$$\tau^8_{\gamma,\delta,w} = \sum_{\epsilon \in A} Z^*_{\epsilon,\delta} \tau^7_{\gamma,\epsilon,w} \quad (2r_D r_T^3) \quad (8856)$$

$$\tau^7_{\gamma,\delta,w} = \sum_{i \in O} \sum_{j \in O} {}^2D^2_{i,w} Y^{2,*}_{i,\delta} \tau^1_{\delta,w,j} \tau^6_{\gamma,i,j} \quad (4r_D r_T^2 N_o^2) \quad (8844)$$

$${}^2R^3_{a,\gamma} \leftarrow \sum_{\delta \in A} \sum_{w \in D} \frac{1}{2} {}^2D^3_{a,w} Y^3_{a,\delta} \tau^0_{\delta,\gamma,w} \tau^8_{\delta,\gamma,w} \quad (4r_D r_T^2 N_v) \quad (8857)$$

$$\tau^8_{\gamma,\delta,w} = \sum_{\epsilon \in A} Z^*_{\epsilon,\delta} \tau^7_{\gamma,\epsilon,w} \quad (2r_D r_T^3) \quad (8845)$$

Raw expression

$${}^2R^3_{a,\gamma} \leftarrow \sum_{\delta \in A} \sum_{w \in D} \frac{1}{2} {}^2D^3_{a,w} Y^1_{a,\delta} \tau^0_{\delta,\gamma,w} \tau^8_{\delta,\gamma,w} \quad (4r_D r_T^2 N_v) \quad (8846)$$

$${}^2R^3_{b,\zeta} \leftarrow \sum_{\gamma \in A} \sum_{i \in O} \sum_{j \in O} \sum_{k \in O} \sum_{l \in O} \sum_{a \in V} \sum_{c \in V} \frac{1}{2} {}^1T_{b,k} Y^{1,*}_{a,\gamma} Y^{2,*}_{i,\gamma} Z^*_{\gamma,\zeta} Y^{4,*}_{j,\zeta} {}^2D^{a,i,b,j} {}^2T_{a,i,c,l} V_{k,c,l,j} \quad (8858)$$

Raw expression

$${}^2R^3_{b,\zeta} \leftarrow \sum_{\gamma \in A} \sum_{i \in O} \sum_{j \in O} \sum_{k \in O} \sum_{l \in O} \sum_{a \in V} \sum_{c \in V} \frac{1}{2} {}^1T_{a,k} Y^{1,*}_{a,\gamma} Y^{2,*}_{i,\gamma} Z^*_{\gamma,\zeta} Y^{4,*}_{j,\zeta} {}^2D^{a,i,b,j} {}^2T_{c,l,b,j} V_{l,i,k,c} \quad (8847)$$

Factorized expression

$$\tau^0_{\gamma,\alpha} = \sum_{a \in V} W^2_{a,\alpha} Y^3_{a,\gamma} \quad (2r_T r_V N_v) \quad (8859)$$

Factorized expression

$$\tau^0_{\gamma,\delta,w} = \sum_{i \in O} {}^2D^4_{i,w} Y^4_{i,\gamma} Y^{4,*}_{i,\delta} \quad (3r_D r_T^2 N_o) \quad (8848)$$

$$\tau^1_{\alpha,i,j} = \sum_{\beta \in B} X_{\alpha,\beta} W^3_{i,\beta} W^4_{j,\beta} \quad (3r_V^2 N_o^2) \quad (8860)$$

$$\tau^1_{\gamma,w,i} = \sum_{a \in V} {}^2D^1_{a,w} {}^1T_{a,i} Y^{1,*}_{a,\gamma} \quad (3r_D r_T N_o N_v) \quad (8849)$$

$$\tau^2_{\gamma,\alpha,i} = \sum_{j \in O} Y^4_{j,\gamma} \tau^1_{\alpha,j,i} \quad (2r_T r_V N_o^2) \quad (8861)$$

$$\tau^3_{\gamma,i,j} = \sum_{\alpha \in B} W^1_{i,\alpha} \tau^0_{\gamma,\alpha} \tau^2_{\gamma,\alpha,j} \quad (3r_T r_V N_o^2) \quad (8862)$$

$$\tau^2_{\alpha,i,j} = \sum_{\beta \in B} W^1_{i,\beta} W^2_{j,\beta} X_{\beta,\alpha} \quad (3r_V^2 N_o^2) \quad (8850)$$

$$\tau^4_{\gamma,i,j} = \sum_{\delta \in A} Z_{\gamma,\delta} \tau^3_{\delta,i,j} \quad (2r_T^2 N_o^2) \quad (8863)$$

$$\tau^3_{\gamma,\alpha,i} = \sum_{j \in O} Y^2_{j,\gamma} \tau^2_{\alpha,j,i} \quad (2r_T r_V N_o^2) \quad (8851)$$

$$\tau^5_{\gamma,\delta,w} = \sum_{a \in V} {}^2D^1_{a,w} Y^1_{a,\gamma} Y^{1,*}_{a,\delta} \quad (3r_D r_T^2 N_v) \quad (8864)$$

$$\tau^4_{\gamma,\alpha} = \sum_{a \in V} W^4_{a,\alpha} Y^1_{a,\gamma} \quad (2r_T r_V N_v) \quad (8852)$$

$$\tau^6_{\gamma,\delta,w} = \sum_{i \in O} {}^2D^2_{i,w} Y^2_{i,\gamma} Y^{2,*}_{i,\delta} \quad (3r_D r_T^2 N_o) \quad (8865)$$

$$\tau^5_{\gamma,i,j} = \sum_{\alpha \in B} W^3_{j,\alpha} \tau^4_{\gamma,\alpha} \tau^3_{\gamma,\alpha,i} \quad (3r_T r_V N_o^2) \quad (8853)$$

$$\tau^7_{\gamma,\delta,w} = \sum_{\epsilon \in A} Z^*_{\epsilon,\delta} \tau^5_{\gamma,\epsilon,w} \tau^6_{\gamma,\epsilon,w} \quad (3r_D r_T^3) \quad (8866)$$

$$\tau_{\gamma,w,i,j}^8 = \sum_{\delta \in A} \tau_{\delta,i,j}^4 \tau_{\delta,\gamma,w}^7 \quad (2r_D r_T^2 N_o^2) \quad (8867)$$

$$\tau_{\gamma,w,i}^9 = \sum_{j \in O} {}^2D_{j,w}^4 Y_{j,\gamma}^{4,*} \tau_{\gamma,w,i,j}^8 \quad (3r_D r_T N_o^2) \quad (8868)$$

$${}^2R_{a,\gamma}^3 \leftarrow \sum_{w \in D} \sum_{i \in O} \frac{1}{2} {}^2D_{a,w}^3 {}^1T_{a,i} \tau_{\gamma,w,i}^9 \quad (3r_D r_T N_o N_v) \quad (8869)$$

Raw expression

$${}^2R_{b,\zeta}^3 \leftarrow \sum_{\gamma \in A} \sum_{i \in O} \sum_{j \in O} \sum_{k \in O} \sum_{l \in O} \sum_{a \in V} \sum_{c \in V} \frac{1}{2} {}^1T_{b,k} Y_{a,\gamma}^{1,*} Y_{i,\gamma}^{2,*} Z_{\gamma,\zeta}^* Y_{j,\zeta}^{4,*} {}^2D_{a,i,b,j} {}^2T_{a,l,c,i} V_{l,c,k,j} \quad (8870)$$

Factorized expression

$$\tau_{\gamma,\alpha}^0 = \sum_{a \in V} W_{a,\alpha}^2 Y_{a,\gamma}^1 \quad (2r_T r_V N_v) \quad (8871)$$

$$\tau_{\alpha,i,j}^1 = \sum_{\beta \in B} X_{\alpha,\beta} W_{i,\beta}^3 W_{j,\beta}^4 \quad (3r_V^2 N_o^2) \quad (8872)$$

$$\tau_{\gamma,\alpha,i}^2 = \sum_{j \in O} Y_{j,\gamma}^2 \tau_{\alpha,j,i}^1 \quad (2r_T r_V N_o^2) \quad (8873)$$

$$\tau_{\gamma,i,j}^3 = \sum_{\alpha \in B} W_{i,\alpha}^1 \tau_{\gamma,\alpha}^0 \tau_{\gamma,\alpha,j}^2 \quad (3r_T r_V N_o^2) \quad (8874)$$

$$\tau_{\gamma,i,j}^4 = \sum_{\delta \in A} Z_{\delta,\gamma} \tau_{\delta,i,j}^3 \quad (2r_T^2 N_o^2) \quad (8875)$$

$$\tau_{\gamma,\delta,w}^5 = \sum_{a \in V} {}^2D_{a,w}^1 Y_{a,\gamma}^3 Y_{a,\delta}^{1,*} \quad (3r_D r_T^2 N_v) \quad (8876)$$

$$\tau_{\gamma,\delta,w}^6 = \sum_{i \in O} {}^2D_{i,w}^2 Y_{i,\gamma}^4 Y_{i,\delta}^{2,*} \quad (3r_D r_T^2 N_o) \quad (8877)$$

$$\tau_{\gamma,\delta,w}^7 = \sum_{\epsilon \in A} Z_{\epsilon,\delta}^* \tau_{\gamma,\epsilon,w}^5 \tau_{\gamma,\epsilon,w}^6 \quad (3r_D r_T^3) \quad (8878)$$

$$\tau_{\gamma,w,i,j}^8 = \sum_{\delta \in A} \tau_{\delta,i,j}^4 \tau_{\delta,\gamma,w}^7 \quad (2r_D r_T^2 N_o^2) \quad (8879)$$

$$\tau_{\gamma,w,i}^9 = \sum_{j \in O} {}^2D_{j,w}^4 Y_{j,\gamma}^{4,*} \tau_{\gamma,w,i,j}^8 \quad (3r_D r_T N_o^2) \quad (8880)$$

$${}^2R_{a,\gamma}^3 \leftarrow \sum_{w \in D} \sum_{i \in O} \frac{1}{2} {}^2D_{a,w}^3 {}^1T_{a,i} \tau_{\gamma,w,i}^9 \quad (3r_D r_T N_o N_v) \quad (8881)$$

Raw expression

$${}^2R_{b,\zeta}^3 \leftarrow \sum_{\gamma \in A} \sum_{i \in O} \sum_{j \in O} \sum_{k \in O} \sum_{l \in O} \sum_{a \in V} \sum_{c \in V} \frac{1}{2} {}^1T_{b,k} Y_{a,\gamma}^{1,*} Y_{i,\gamma}^{2,*} Z_{\gamma,\zeta}^* Y_{j,\zeta}^{4,*} {}^2D_{a,i,b,j} {}^2T_{a,l,c,j} V_{l,i,k,c} \quad (8882)$$

Factorized expression

$$\tau_{\gamma,\delta,w}^0 = \sum_{a \in V} {}^2D_{a,w}^1 Y_{a,\gamma}^1 Y_{a,\delta}^{1,*} \quad (3r_D r_T^2 N_v) \quad (8883)$$

$$\tau_{\gamma,\alpha}^1 = \sum_{i \in O} W_{i,\alpha}^1 Y_{i,\gamma}^2 \quad (2r_T r_V N_o) \quad (8884)$$

$$\tau_{\gamma,\alpha}^2 = \sum_{a \in V} W_{a,\alpha}^2 Y_{a,\gamma}^3 \quad (2r_T r_V N_v) \quad (8885)$$

$$\tau_{\gamma,\alpha,i}^3 = \sum_{\delta \in A} Z_{\gamma,\delta} Y_{i,\delta}^4 \tau_{\delta,\alpha}^2 \quad (3r_T^2 r_V N_o) \quad (8886)$$

$$\tau_{\gamma,\alpha,w}^4 = \sum_{\delta \in A} \sum_{i \in O} {}^2D_{i,w}^2 Y_{i,\gamma}^{2,*} \tau_{\delta,\alpha}^1 \tau_{\delta,\gamma,w}^0 \tau_{\delta,\alpha,i}^3 \quad (5r_D r_T^2 r_V N_o) \quad (8887)$$

$$\tau_{\gamma,\alpha,w}^5 = \sum_{\beta \in B} X_{\beta,\alpha} \tau_{\gamma,\beta,w}^4 \quad (2r_D r_T r_V^2) \quad (8888)$$

$$\tau_{\gamma,\alpha,w}^6 = \sum_{\delta \in A} Z_{\delta,\gamma}^* \tau_{\delta,\alpha,w}^5 \quad (2r_D r_T^2 r_V) \quad (8889)$$

$$\tau_{\gamma,\alpha,w}^7 = \sum_{i \in O} {}^2D_{i,w}^4 W_{i,\alpha}^4 Y_{i,\gamma}^{4,*} \quad (3r_D r_T r_V N_o) \quad (8890)$$

$$\tau_{\gamma,w,i}^8 = \sum_{\alpha \in B} W_{i,\alpha}^3 \tau_{\gamma,\alpha,w}^6 \tau_{\gamma,\alpha,w}^7 \quad (3r_D r_T r_V N_o) \quad (8891)$$

$${}^2R^3_{a,\gamma} \leftarrow \sum_{w \in D} \sum_{i \in O} \frac{1}{2} {}^2D^3_{a,w} {}^1T_{a,i} \tau^8_{\gamma,w,i} \quad (3r_D r_T N_o N_v) \quad (8892)$$

Raw expression

$${}^2R^3_{b,\zeta} \leftarrow \sum_{\gamma \in A} \sum_{i \in O} \sum_{j \in O} \sum_{k \in O} \sum_{l \in O} \sum_{a \in V} \sum_{c \in V} \frac{1}{2} {}^1T_{b,k} Y^{1,*}_{a,\gamma} Y^{2,*}_{i,\gamma} Z^*_{\gamma,\zeta} Y^{4,*}_{j,\zeta} {}^2D^{a,i,b,j} {}^2T_{c,i,a,l} V_{l,c,k,j} \quad (8893)$$

Factorized expression

$$\tau^0_{\gamma,\delta,w} = \sum_{a \in V} {}^2D^1_{a,w} Y^3_{a,\gamma} Y^{1,*}_{a,\delta} \quad (3r_D r_T^2 N_v) \quad (8894)$$

$$\tau^1_{\gamma,\alpha} = \sum_{a \in V} W^2_{a,\alpha} Y^1_{a,\gamma} \quad (2r_T r_V N_v) \quad (8895)$$

$$\tau^2_{\gamma,\alpha,i} = \sum_{\delta \in A} Y^2_{i,\delta} Z_{\delta,\gamma} \tau^1_{\delta,\alpha} \quad (3r_T^2 r_V N_o) \quad (8896)$$

$$\tau^3_{\gamma,\alpha} = \sum_{i \in O} W^1_{i,\alpha} Y^4_{i,\gamma} \quad (2r_T r_V N_o) \quad (8897)$$

$$\tau^4_{\gamma,\alpha,w} = \sum_{\delta \in A} \sum_{i \in O} {}^2D^2_{i,w} Y^{2,*}_{i,\gamma} \tau^3_{\delta,\alpha} \tau^0_{\delta,\gamma,w} \tau^2_{\delta,\alpha,i} \quad (5r_D r_T^2 r_V N_o) \quad (8898)$$

$$\tau^5_{\gamma,\alpha,w} = \sum_{\beta \in B} X_{\beta,\alpha} \tau^4_{\gamma,\beta,w} \quad (2r_D r_T r_V^2) \quad (8899)$$

$$\tau^6_{\gamma,\alpha,w} = \sum_{\delta \in A} Z^*_{\delta,\gamma} \tau^5_{\delta,\alpha,w} \quad (2r_D r_T^2 r_V) \quad (8900)$$

$$\tau^7_{\gamma,\alpha,w} = \sum_{i \in O} {}^2D^4_{i,w} W^4_{i,\alpha} Y^{4,*}_{i,\gamma} \quad (3r_D r_T r_V N_o) \quad (8901)$$

$$\tau^8_{\gamma,w,i} = \sum_{\alpha \in B} W^3_{i,\alpha} \tau^6_{\gamma,\alpha,w} \tau^7_{\gamma,\alpha,w} \quad (3r_D r_T r_V N_o) \quad (8902)$$

$${}^2R^3_{a,\gamma} \leftarrow \sum_{w \in D} \sum_{i \in O} \frac{1}{2} {}^2D^3_{a,w} {}^1T_{a,i} \tau^8_{\gamma,w,i} \quad (3r_D r_T N_o N_v) \quad (8903)$$

Raw expression

$${}^2R^3_{b,\zeta} \leftarrow \sum_{\gamma \in A} \sum_{i \in O} \sum_{j \in O} \sum_{k \in O} \sum_{l \in O} \sum_{a \in V} \sum_{c \in V} \frac{1}{2} {}^1T_{b,k} Y^{1,*}_{a,\gamma} Y^{2,*}_{i,\gamma} Z^*_{\gamma,\zeta} Y^{4,*}_{j,\zeta} {}^2D^{a,i,b,j} {}^2T_{c,j,a,l} V_{l,i,k,c} \quad (8904)$$

Factorized expression

$$\tau^0_{\gamma,\delta,w} = \sum_{a \in V} {}^2D^1_{a,w} Y^1_{a,\gamma} Y^{1,*}_{a,\delta} \quad (3r_D r_T^2 N_v) \quad (8905)$$

$$\tau^1_{\alpha,i,j} = \sum_{\beta \in B} W^1_{i,\beta} W^2_{j,\beta} X_{\beta,\alpha} \quad (3r_V^2 N_o^2) \quad (8906)$$

$$\tau^2_{\gamma,\alpha,i} = \sum_{j \in O} Y^2_{j,\gamma} \tau^1_{\alpha,j,i} \quad (2r_T r_V N_o^2) \quad (8907)$$

$$\tau^3_{\gamma,\delta,\alpha,w} = \sum_{i \in O} {}^2D^2_{i,w} Y^{2,*}_{i,\delta} \tau^0_{\gamma,\delta,w} \tau^2_{\gamma,\alpha,i} \quad (4r_D r_T^2 r_V N_o) \quad (8908)$$

$$\tau^4_{\gamma,\alpha} = \sum_{a \in V} W^4_{a,\alpha} Y^3_{a,\gamma} \quad (2r_T r_V N_v) \quad (8909)$$

$$\tau^5_{\gamma,\alpha,i} = \sum_{\delta \in A} Z_{\gamma,\delta} Y^4_{i,\delta} \tau^4_{\delta,\alpha} \quad (3r_T^2 r_V N_o) \quad (8910)$$

$$\tau^6_{\gamma,\alpha,w,i} = \sum_{\delta \in A} \tau^5_{\delta,\alpha,i} \tau^3_{\delta,\gamma,\alpha,w} \quad (2r_D r_T^2 r_V N_o) \quad (8911)$$

$$\tau^7_{\gamma,w,i,j} = \sum_{\alpha \in B} W^3_{i,\alpha} \tau^6_{\gamma,\alpha,w,j} \quad (2r_D r_T r_V N_o^2) \quad (8912)$$

$$\tau^8_{\gamma,w,i} = \sum_{\delta \in A} \sum_{j \in O} {}^2D^4_{j,w} Z^*_{\delta,\gamma} Y^{4,*}_{j,\gamma} \tau^7_{\delta,w,i,j} \quad (4r_D r_T^2 N_o^2) \quad (8913)$$

$${}^2R^3_{a,\gamma} \leftarrow \sum_{w \in D} \sum_{i \in O} \frac{1}{2} {}^2D^3_{a,w} {}^1T_{a,i} \tau^8_{\gamma,w,i} \quad (3r_D r_T N_o N_v) \quad (8914)$$

Raw expression

$${}^2R^3_{b,\zeta} \leftarrow \sum_{\gamma \in A} \sum_{i \in O} \sum_{j \in O} \sum_{k \in O} \sum_{l \in O} \sum_{a \in V} \sum_{c \in V} \frac{1}{2} {}^1T_{b,k} Y^{1,*}_{a,\gamma} Y^{2,*}_{i,\gamma} Z^*_{\gamma,\zeta} Y^{4,*}_{j,\zeta} {}^2D^{a,i,b,j} {}^2T_{c,l,a,i} V_{k,c,l,j} \quad (8915)$$

Factorized expression

$$\tau^0_{\gamma,\delta,w} = \sum_{a \in V} {}^2D^1_{a,w} Y^3_{a,\gamma} Y^{1,*}_{a,\delta} \quad (3r_D r_T^2 N_v) \quad (8916)$$

$$\tau^1_{\alpha,i,j} = \sum_{\beta \in B} W^1_{i,\beta} W^2_{j,\beta} X_{\beta,\alpha} \quad (3r_V^2 N_o^2) \quad (8917)$$

$$\tau^2_{\gamma,\alpha,i} = \sum_{j \in O} Y^4_{j,\gamma} \tau^1_{\alpha,j,i} \quad (2r_T r_V N_o^2) \quad (8918)$$

$$\tau^3_{\gamma,\delta,\alpha,w} = \sum_{i \in O} {}^2D^2_{i,w} Y^{2,*}_{i,\delta} \tau^0_{\gamma,\delta,w} \tau^2_{\gamma,\alpha,i} \quad (4r_D r_T^2 r_V N_o) \quad (8919)$$

$$\tau^4_{\gamma,\alpha} = \sum_{a \in V} W^4_{a,\alpha} Y^1_{a,\gamma} \quad (2r_T r_V N_v) \quad (8920)$$

$$\tau^5_{\gamma,\alpha,i} = \sum_{\delta \in A} Y^2_{i,\delta} Z_{\delta,\gamma} \tau^4_{\delta,\alpha} \quad (3r_T^2 r_V N_o) \quad (8921)$$

$$\tau^6_{\gamma,\alpha,w,i} = \sum_{\delta \in A} \tau^5_{\delta,\alpha,i} \tau^3_{\delta,\gamma,\alpha,w} \quad (2r_D r_T^2 r_V N_o) \quad (8922)$$

$$\tau^7_{\gamma,w,i,j} = \sum_{\alpha \in B} W^3_{i,\alpha} \tau^6_{\gamma,\alpha,w,j} \quad (2r_D r_T r_V N_o^2) \quad (8923)$$

$$\tau^8_{\gamma,w,i} = \sum_{\delta \in A} \sum_{j \in O} {}^2D^4_{j,w} Z^*_{\delta,\gamma} Y^{4,*}_{j,\gamma} \tau^7_{\delta,w,i,j} \quad (4r_D r_T^2 N_o^2) \quad (8924)$$

$${}^2R^3_{a,\gamma} \leftarrow \sum_{w \in D} \sum_{i \in O} \frac{1}{2} {}^2D^3_{a,w} {}^1T_{a,i} \tau^8_{\gamma,w,i} \quad (3r_D r_T N_o N_v) \quad (8925)$$

Raw expression

$${}^2R^3_{b,\zeta} \leftarrow \sum_{\gamma \in A} \sum_{i \in O} \sum_{j \in O} \sum_{k \in O} \sum_{l \in O} \sum_{a \in V} \sum_{c \in V} \frac{1}{2} {}^1T_{c,i} Y^{1,*}_{a,\gamma} Y^{2,*}_{i,\gamma} Z^*_{\gamma,\zeta} Y^{4,*}_{j,\zeta} {}^2D^{a,i,b,j} {}^2T_{a,k,b,l} V_{k,c,l,j} \quad (8926)$$

Factorized expression

$$\tau^0_{\alpha,i} = \sum_{a \in V} {}^1T_{a,i} W^2_{a,\alpha} \quad (2r_V N_o N_v) \quad (8927)$$

$$\tau^1_{\gamma,\alpha,w} = \sum_{i \in O} {}^2D^2_{i,w} Y^{2,*}_{i,\gamma} \tau^0_{\alpha,i} \quad (3r_D r_T r_V N_o) \quad (8928)$$

$$\tau^2_{\gamma,\delta,w} = \sum_{a \in V} {}^2D^1_{a,w} Y^1_{a,\gamma} Y^{1,*}_{a,\delta} \quad (3r_D r_T^2 N_v) \quad (8929)$$

$$\tau^3_{\gamma,\delta,w,i} = \sum_{\epsilon \in A} Y^2_{i,\epsilon} Z_{\epsilon,\gamma} \tau^2_{\epsilon,\delta,w} \quad (3r_D r_T^3 N_o) \quad (8930)$$

$$\tau^4_{\gamma,\delta,\alpha,w} = \sum_{i \in O} W^1_{i,\alpha} \tau^1_{\delta,\alpha,w} \tau^3_{\gamma,\delta,w,i} \quad (3r_D r_T^2 r_V N_o) \quad (8931)$$

$$\tau^5_{\alpha,i,j} = \sum_{\beta \in B} X_{\alpha,\beta} W^3_{i,\beta} W^4_{j,\beta} \quad (3r_V^2 N_o^2) \quad (8932)$$

$$\tau^6_{\gamma,\alpha,i} = \sum_{j \in O} Y^4_{j,\gamma} \tau^5_{\alpha,j,i} \quad (2r_T r_V N_o^2) \quad (8933)$$

$$\tau^7_{\gamma,\delta,w,i} = \sum_{\alpha \in B} \tau^6_{\gamma,\alpha,i} \tau^4_{\gamma,\delta,\alpha,w} \quad (2r_D r_T^2 r_V N_o) \quad (8934)$$

$$\tau^8_{\gamma,\delta,w} = \sum_{\epsilon \in A} \sum_{i \in O} {}^2D^4_{i,w} Z^*_{\epsilon,\delta} Y^{4,*}_{i,\delta} \tau^7_{\gamma,\epsilon,w,i} \quad (4r_D r_T^3 N_o) \quad (8935)$$

$${}^2R^3_{a,\gamma} \leftarrow \sum_{\delta \in A} \sum_{w \in D} \frac{1}{2} {}^2D^3_{a,w} Y^3_{a,\delta} \tau^8_{\delta,\gamma,w} \quad (3r_D r_T^2 N_v) \quad (8936)$$

Raw expression

$${}^2R^3_{b,\zeta} \leftarrow \sum_{\gamma \in A} \sum_{i \in O} \sum_{j \in O} \sum_{k \in O} \sum_{l \in O} \sum_{a \in V} \sum_{c \in V} \frac{1}{2} {}^1T_{c,i} Y^{1,*}_{a,\gamma} Y^{2,*}_{i,\gamma} Z^*_{\gamma,\zeta} Y^{4,*}_{j,\zeta} {}^2D^{a,i,b,j} {}^2T_{b,k,a,l} V_{l,c,k,j} \quad (8937)$$

Factorized expression

$$\tau^0_{\alpha,i} = \sum_{a \in V} {}^1T_{a,i} W^2_{a,\alpha} \quad (2r_V N_o N_v) \quad (8938)$$

$$\tau^1_{\gamma,\alpha,w} = \sum_{i \in O} {}^2D^2_{i,w} Y^{2,*}_{i,\gamma} \tau^0_{\alpha,i} \quad (3r_D r_T r_V N_o) \quad (8939)$$

$$\tau^2_{\gamma,\delta,w} = \sum_{a \in V} {}^2D^1_{a,w} Y^3_{a,\gamma} Y^{1,*}_{a,\delta} \quad (3r_D r_T^2 N_v) \quad (8940)$$

$$\tau^3_{\gamma,\delta,w,i} = \sum_{\epsilon \in A} Z_{\gamma,\epsilon} Y^4_{i,\epsilon} \tau^2_{\epsilon,\delta,w} \quad (3r_D r_T^3 N_o) \quad (8941)$$

$$\tau^4_{\alpha,i} = \sum_{a \in V} {}^1T_{a,i} W^4_{a,\alpha} \quad (2r_V N_o N_v) \quad (8953)$$

$$\tau^4_{\gamma,\delta,\alpha,w} = \sum_{i \in O} W^1_{i,\alpha} \tau^1_{\delta,\alpha,w} \tau^3_{\gamma,\delta,w,i} \quad (3r_D r_T^2 r_V N_o) \quad (8942)$$

$$\tau^5_{\alpha,i,j} = \sum_{\beta \in B} X_{\alpha,\beta} W^3_{j,\beta} \tau^4_{\beta,i} \quad (3r_V^2 N_o^2) \quad (8954)$$

$$\tau^5_{\alpha,i,j} = \sum_{\beta \in B} X_{\alpha,\beta} W^3_{i,\beta} W^4_{j,\beta} \quad (3r_V^2 N_o^2) \quad (8943)$$

$$\tau^6_{\gamma,\alpha,i} = \sum_{j \in O} Y^4_{j,\gamma} \tau^5_{\alpha,i,j} \quad (2r_T r_V N_o^2) \quad (8955)$$

$$\tau^6_{\gamma,\alpha,i} = \sum_{j \in O} Y^2_{j,\gamma} \tau^5_{\alpha,j,i} \quad (2r_T r_V N_o^2) \quad (8944)$$

$$\tau^7_{\gamma,\delta,w,i} = \sum_{\alpha \in B} \tau^6_{\gamma,\alpha,i} \tau^3_{\gamma,\delta,\alpha,w} \quad (2r_D r_T^2 r_V N_o) \quad (8956)$$

$$\tau^7_{\gamma,\delta,w,i} = \sum_{\alpha \in B} \tau^6_{\gamma,\alpha,i} \tau^4_{\gamma,\delta,\alpha,w} \quad (2r_D r_T^2 r_V N_o) \quad (8945)$$

$$\tau^8_{\gamma,\delta,w} = \sum_{\epsilon \in A} \sum_{i \in O} {}^2D^4_{i,w} Z^*_{\epsilon,\delta} Y^{4,*}_{i,\delta} \tau^7_{\gamma,\epsilon,w,i} \quad (4r_D r_T^3 N_o) \quad (8957)$$

$$\tau^8_{\gamma,\delta,w} = \sum_{\epsilon \in A} \sum_{i \in O} {}^2D^4_{i,w} Z^*_{\epsilon,\delta} Y^{4,*}_{i,\delta} \tau^7_{\gamma,\epsilon,w,i} \quad (4r_D r_T^3 N_o) \quad (8946)$$

$${}^2R^3_{a,\gamma} \leftarrow \sum_{\delta \in A} \sum_{w \in D} \frac{1}{2} {}^2D^3_{a,w} Y^3_{a,\delta} \tau^8_{\delta,\gamma,w} \quad (3r_D r_T^2 N_v) \quad (8958)$$

$${}^2R^3_{a,\gamma} \leftarrow \sum_{\delta \in A} \sum_{w \in D} \frac{1}{2} {}^2D^3_{a,w} Y^1_{a,\delta} \tau^8_{\delta,\gamma,w} \quad (3r_D r_T^2 N_v) \quad (8947)$$

Raw expression

$${}^2R^3_{b,\zeta} \leftarrow \sum_{\gamma \in A} \sum_{i \in O} \sum_{j \in O} \sum_{k \in O} \sum_{l \in O} \sum_{a \in V} \sum_{c \in V} \frac{1}{2} {}^1T_{c,j} Y^{1,*}_{a,\gamma} Y^{2,*}_{i,\gamma} Z^*_{\gamma,\zeta} Y^{4,*}_{j,\zeta} {}^2D^{a,i,b,j} {}^2T_{b,k,a,l} V_{l,i,k,c} \quad (8959)$$

Raw expression

$${}^2R^3_{b,\zeta} \leftarrow \sum_{\gamma \in A} \sum_{i \in O} \sum_{j \in O} \sum_{k \in O} \sum_{l \in O} \sum_{a \in V} \sum_{c \in V} \frac{1}{2} {}^1T_{c,j} Y^{1,*}_{a,\gamma} Y^{2,*}_{i,\gamma} Z^*_{\gamma,\zeta} Y^{4,*}_{j,\zeta} {}^2D^{a,i,b,j} {}^2T_{a,k,b,l} V_{k,i,l,c} \quad (8948)$$

Factorized expression

$$\tau^0_{\gamma,\alpha,w} = \sum_{i \in O} {}^2D^2_{i,w} W^2_{i,\alpha} Y^{2,*}_{i,\gamma} \quad (3r_D r_T r_V N_o) \quad (8960)$$

$$\tau^0_{\gamma,\alpha,w} = \sum_{i \in O} {}^2D^2_{i,w} W^2_{i,\alpha} Y^{2,*}_{i,\gamma} \quad (3r_D r_T r_V N_o) \quad (8949)$$

$$\tau^1_{\gamma,\delta,w} = \sum_{a \in V} {}^2D^1_{a,w} Y^3_{a,\gamma} Y^{1,*}_{a,\delta} \quad (3r_D r_T^2 N_v) \quad (8961)$$

$$\tau^1_{\gamma,\delta,w} = \sum_{a \in V} {}^2D^1_{a,w} Y^1_{a,\gamma} Y^{1,*}_{a,\delta} \quad (3r_D r_T^2 N_v) \quad (8950)$$

$$\tau^2_{\gamma,\delta,w,i} = \sum_{\epsilon \in A} Z_{\gamma,\epsilon} Y^4_{i,\epsilon} \tau^1_{\epsilon,\delta,w} \quad (3r_D r_T^3 N_o) \quad (8962)$$

$$\tau^2_{\gamma,\delta,w,i} = \sum_{\epsilon \in A} Y^2_{i,\epsilon} Z_{\epsilon,\gamma} \tau^1_{\epsilon,\delta,w} \quad (3r_D r_T^3 N_o) \quad (8951)$$

$$\tau^3_{\gamma,\delta,\alpha,w} = \sum_{i \in O} W^1_{i,\alpha} \tau^0_{\delta,\alpha,w} \tau^2_{\gamma,\delta,w,i} \quad (3r_D r_T^2 r_V N_o) \quad (8963)$$

$$\tau^3_{\gamma,\delta,\alpha,w} = \sum_{i \in O} W^1_{i,\alpha} \tau^0_{\delta,\alpha,w} \tau^2_{\gamma,\delta,w,i} \quad (3r_D r_T^2 r_V N_o) \quad (8952)$$

$$\tau^4_{\alpha,i} = \sum_{a \in V} {}^1T_{a,i} W^4_{a,\alpha} \quad (2r_V N_o N_v) \quad (8964)$$



$$\tau^5_{\alpha,i,j} = \sum_{\beta \in B} X_{\alpha,\beta} W^3_{j,\beta} \tau^4_{\beta,i} \quad (3r_V^2 N_o^2) \quad (8965)$$

$$\tau^7_{\gamma,\delta,w} = \sum_{i \in O} {}^2D^2_{i,w} Y^{2,*}_{i,\delta} \tau^6_{\gamma,i} \quad (3r_D r_T^2 N_o) \quad (8978)$$

$$\tau^6_{\gamma,\alpha,i} = \sum_{j \in O} Y^2_{j,\gamma} \tau^5_{\alpha,i,j} \quad (2r_T r_V N_o^2) \quad (8966)$$

$$\tau^8_{\gamma,\delta,w} = \sum_{\epsilon \in A} Z^*_{\epsilon,\delta} \tau^1_{\gamma,\epsilon,w} \tau^7_{\gamma,\epsilon,w} \quad (3r_D r_T^3) \quad (8979)$$

$$\tau^7_{\gamma,\delta,w,i} = \sum_{\alpha \in B} \tau^6_{\gamma,\alpha,i} \tau^3_{\gamma,\delta,\alpha,w} \quad (2r_D r_T^2 r_V N_o) \quad (8967)$$

$$\tau^9_{\gamma,\delta,w} = \sum_{\epsilon \in A} Z_{\epsilon,\gamma} \tau^8_{\epsilon,\delta,w} \quad (2r_D r_T^3) \quad (8980)$$

$$\tau^8_{\gamma,\delta,w} = \sum_{\epsilon \in A} \sum_{i \in O} {}^2D^4_{i,w} Z^*_{\epsilon,\delta} Y^{4,*}_{i,\delta} \tau^7_{\gamma,\epsilon,w,i} \quad (4r_D r_T^3 N_o) \quad (8968)$$

$${}^2R^3_{a,\gamma} \leftarrow \sum_{\delta \in A} \sum_{w \in D} \frac{1}{2} {}^2D^3_{a,w} Y^3_{a,\delta} \tau^0_{\delta,\gamma,w} \tau^9_{\delta,\gamma,w} \quad (4r_D r_T^2 N_v) \quad (8981)$$

$${}^2R^3_{a,\gamma} \leftarrow \sum_{\delta \in A} \sum_{w \in D} \frac{1}{2} {}^2D^3_{a,w} Y^1_{a,\delta} \tau^8_{\delta,\gamma,w} \quad (3r_D r_T^2 N_v) \quad (8969)$$

Raw expression

$${}^2R^3_{b,\zeta} \leftarrow \sum_{\gamma \in A} \sum_{i \in O} \sum_{j \in O} \sum_{k \in O} \sum_{l \in O} \sum_{a \in V} \sum_{c \in V} \frac{1}{2} {}^1T_{c,k} Y^{1,*}_{a,\gamma} Y^{2,*}_{i,\gamma} Z^*_{\gamma,\zeta} Y^{4,*}_{j,\zeta} {}^2D^{a,i,b,j} {}^2T_{a,l,b,j} V_{k,i,l,c} \quad (8982)$$

Raw expression

$${}^2R^3_{b,\zeta} \leftarrow \sum_{\gamma \in A} \sum_{i \in O} \sum_{j \in O} \sum_{k \in O} \sum_{l \in O} \sum_{a \in V} \sum_{c \in V} \frac{1}{2} {}^1T_{c,k} Y^{1,*}_{a,\gamma} Y^{2,*}_{i,\gamma} Z^*_{\gamma,\zeta} Y^{4,*}_{j,\zeta} {}^2D^{a,i,b,j} {}^2T_{a,i,b,l} V_{l,c,k,j} \quad (8970)$$

Factorized expression

$$\tau^0_{\gamma,\delta,w} = \sum_{i \in O} {}^2D^4_{i,w} Y^2_{i,\gamma} Y^{4,*}_{i,\delta} \quad (3r_D r_T^2 N_o) \quad (8983)$$

Factorized expression

$$\tau^0_{\gamma,\delta,w} = \sum_{i \in O} {}^2D^4_{i,w} Y^4_{i,\gamma} Y^{4,*}_{i,\delta} \quad (3r_D r_T^2 N_o) \quad (8971)$$

$$\tau^1_{\gamma,\delta,w} = \sum_{a \in V} {}^2D^1_{a,w} Y^3_{a,\gamma} Y^{1,*}_{a,\delta} \quad (3r_D r_T^2 N_v) \quad (8984)$$

$$\tau^1_{\gamma,\delta,w} = \sum_{a \in V} {}^2D^1_{a,w} Y^1_{a,\gamma} Y^{1,*}_{a,\delta} \quad (3r_D r_T^2 N_v) \quad (8972)$$

$$\tau^2_{\alpha,i} = \sum_{a \in V} {}^1T_{a,i} W^4_{a,\alpha} \quad (2r_V N_o N_v) \quad (8985)$$

$$\tau^2_{\alpha,i} = \sum_{a \in V} {}^1T_{a,i} W^4_{a,\alpha} \quad (2r_V N_o N_v) \quad (8973)$$

$$\tau^3_{\alpha,\beta} = \sum_{i \in O} W^1_{i,\alpha} \tau^2_{\beta,i} \quad (2r_V^2 N_o) \quad (8986)$$

$$\tau^3_{\alpha,\beta} = \sum_{i \in O} W^1_{i,\alpha} \tau^2_{\beta,i} \quad (2r_V^2 N_o) \quad (8974)$$

$$\tau^4_{\alpha,i} = \sum_{\beta \in B} X_{\alpha,\beta} W^3_{i,\beta} \tau^3_{\alpha,\beta} \quad (3r_V^2 N_o) \quad (8987)$$

$$\tau^4_{\alpha,i} = \sum_{\beta \in B} X_{\alpha,\beta} W^3_{i,\beta} \tau^3_{\alpha,\beta} \quad (3r_V^2 N_o) \quad (8975)$$

$$\tau^5_{i,j} = \sum_{\alpha \in B} W^2_{i,\alpha} \tau^4_{\alpha,j} \quad (2r_V N_o^2) \quad (8988)$$

$$\tau^5_{i,j} = \sum_{\alpha \in B} W^2_{i,\alpha} \tau^4_{\alpha,j} \quad (2r_V N_o^2) \quad (8976)$$

$$\tau^6_{\gamma,i} = \sum_{j \in O} Y^4_{j,\gamma} \tau^5_{i,j} \quad (2r_T N_o^2) \quad (8989)$$

$$\tau^6_{\gamma,i} = \sum_{j \in O} Y^2_{j,\gamma} \tau^5_{i,j} \quad (2r_T N_o^2) \quad (8977)$$

$$\tau^7_{\gamma,\delta,w} = \sum_{i \in O} {}^2D^2_{i,w} Y^{2,*}_{i,\delta} \tau^6_{\gamma,i} \quad (3r_D r_T^2 N_o) \quad (8990)$$

$$\tau_{\gamma,\delta,w}^8 = \sum_{\epsilon \in A} Z_{\epsilon,\delta}^* \tau_{\gamma,\epsilon,w}^1 \tau_{\gamma,\epsilon,w}^7 \quad (3r_D r_T^3) \quad (8991)$$

$$\tau_{\gamma,\delta,w}^9 = \sum_{\epsilon \in A} Z_{\epsilon,\gamma} \tau_{\epsilon,\delta,w}^8 \quad (2r_D r_T^3) \quad (9004)$$

$$\tau_{\gamma,\delta,w}^9 = \sum_{\epsilon \in A} Z_{\gamma,\epsilon} \tau_{\epsilon,\delta,w}^8 \quad (2r_D r_T^3) \quad (8992)$$

$${}^2R_{a,\gamma}^3 \leftarrow \sum_{\delta \in A} \sum_{w \in D} \frac{1}{2} {}^2D_{a,w}^3 Y_{a,\delta}^3 \tau_{\delta,\gamma,w}^5 \tau_{\delta,\gamma,w}^9 \quad (4r_D r_T^2 N_v) \quad (9005)$$

$${}^2R_{a,\gamma}^3 \leftarrow \sum_{\delta \in A} \sum_{w \in D} \frac{1}{2} {}^2D_{a,w}^3 Y_{a,\delta}^1 \tau_{\delta,\gamma,w}^0 \tau_{\delta,\gamma,w}^9 \quad (4r_D r_T^2 N_v) \quad \text{Raw expression} \quad (8993)$$

Raw expression

$${}^2R_{b,\zeta}^3 \leftarrow \sum_{\gamma \in A} \sum_{i \in O} \sum_{j \in O} \sum_{k \in O} \sum_{l \in O} \sum_{a \in V} \sum_{c \in V} \frac{1}{2} {}^1T_{c,k} Y_{a,\gamma}^{1,*} Y_{i,\gamma}^{2,*} Z_{\gamma,\zeta}^* Y_{j,\zeta}^{4,*} {}^2D_{a,i,b,j} {}^2T_{b,l,a,i} V_{l,c,k,j} \quad (9006)$$

$${}^2R_{b,\zeta}^3 \leftarrow \sum_{\gamma \in A} \sum_{i \in O} \sum_{j \in O} \sum_{k \in O} \sum_{l \in O} \sum_{a \in V} \sum_{c \in V} \frac{1}{2} {}^1T_{c,k} Y_{a,\gamma}^{1,*} Y_{i,\gamma}^{2,*} Z_{\gamma,\zeta}^* Y_{j,\zeta}^{4,*} {}^2D_{a,i,b,j} {}^2T_{b,j,a,l} V_{k,i,l,c} \quad (8994)$$

Factorized expression

Factorized expression

$$\tau_{\alpha,i}^0 = \sum_{a \in V} {}^1T_{a,i} W_{a,\alpha}^2 \quad (2r_V N_o N_v) \quad (9007)$$

$$\tau_{\alpha,i}^0 = \sum_{a \in V} {}^1T_{a,i} W_{a,\alpha}^2 \quad (2r_V N_o N_v) \quad (8995)$$

$$\tau_{\alpha,\beta}^1 = \sum_{i \in O} W_{i,\beta}^3 \tau_{\alpha,i}^0 \quad (2r_V^2 N_o) \quad (9008)$$

$$\tau_{\alpha,\beta}^1 = \sum_{i \in O} W_{i,\beta}^3 \tau_{\alpha,i}^0 \quad (2r_V^2 N_o) \quad (8996)$$

$$\tau_{\alpha,i}^2 = \sum_{\beta \in B} X_{\alpha,\beta} W_{i,\beta}^4 \tau_{\alpha,\beta}^1 \quad (3r_V^2 N_o) \quad (9009)$$

$$\tau_{\alpha,i}^2 = \sum_{\beta \in B} X_{\alpha,\beta} W_{i,\beta}^4 \tau_{\alpha,\beta}^1 \quad (3r_V^2 N_o) \quad (8997)$$

$$\tau_{i,j}^3 = \sum_{\alpha \in B} W_{i,\alpha}^1 \tau_{\alpha,j}^2 \quad (2r_V N_o^2) \quad (9010)$$

$$\tau_{i,j}^3 = \sum_{\alpha \in B} W_{i,\alpha}^1 \tau_{\alpha,j}^2 \quad (2r_V N_o^2) \quad (8998)$$

$$\tau_{\gamma,i}^4 = \sum_{j \in O} Y_{j,\gamma}^2 \tau_{j,i}^3 \quad (2r_T N_o^2) \quad (9011)$$

$$\tau_{\gamma,i}^4 = \sum_{j \in O} Y_{j,\gamma}^4 \tau_{j,i}^3 \quad (2r_T N_o^2) \quad (8999)$$

$$\tau_{\gamma,\delta,w}^5 = \sum_{i \in O} {}^2D_{i,w}^4 Y_{i,\delta}^{4,*} \tau_{\gamma,i}^4 \quad (3r_D r_T^2 N_o) \quad (9012)$$

$$\tau_{\gamma,\delta,w}^5 = \sum_{i \in O} {}^2D_{i,w}^4 Y_{i,\delta}^{4,*} \tau_{\gamma,i}^4 \quad (3r_D r_T^2 N_o) \quad (9000)$$

$$\tau_{\gamma,\delta,w}^6 = \sum_{a \in V} {}^2D_{a,w}^1 Y_{a,\gamma}^3 Y_{a,\delta}^{1,*} \quad (3r_D r_T^2 N_v) \quad (9013)$$

$$\tau_{\gamma,\delta,w}^6 = \sum_{a \in V} {}^2D_{a,w}^1 Y_{a,\gamma}^1 Y_{a,\delta}^{1,*} \quad (3r_D r_T^2 N_v) \quad (9001)$$

$$\tau_{\gamma,\delta,w}^7 = \sum_{i \in O} {}^2D_{i,w}^2 Y_{i,\gamma}^4 Y_{i,\delta}^{2,*} \quad (3r_D r_T^2 N_o) \quad (9014)$$

$$\tau_{\gamma,\delta,w}^7 = \sum_{i \in O} {}^2D_{i,w}^2 Y_{i,\gamma}^2 Y_{i,\delta}^{2,*} \quad (3r_D r_T^2 N_o) \quad (9002)$$

$$\tau_{\gamma,\delta,w}^8 = \sum_{\epsilon \in A} Z_{\epsilon,\delta}^* \tau_{\gamma,\epsilon,w}^6 \tau_{\gamma,\epsilon,w}^7 \quad (3r_D r_T^3) \quad (9015)$$

$$\tau_{\gamma,\delta,w}^8 = \sum_{\epsilon \in A} Z_{\epsilon,\delta}^* \tau_{\gamma,\epsilon,w}^6 \tau_{\gamma,\epsilon,w}^7 \quad (3r_D r_T^3) \quad (9003)$$

$$\tau_{\gamma,\delta,w}^9 = \sum_{\epsilon \in A} Z_{\gamma,\epsilon} \tau_{\epsilon,\delta,w}^8 \quad (2r_D r_T^3) \quad (9016)$$

Raw expression

$${}^2R^3_{a,\gamma} \leftarrow \sum_{\delta \in A} \sum_{w \in D} \frac{1}{2} {}^2D^3_{a,w} Y^1_{a,\delta} \tau^5_{\delta,\gamma,w} \tau^9_{\delta,\gamma,w} \quad (4r_D r_T^2 N_v) \quad (9017)$$

$${}^2R^3_{b,\zeta} \leftarrow - \sum_{\gamma \in A} \sum_{i \in O} \sum_{j \in O} \sum_{k \in O} \sum_{l \in O} \sum_{a \in V} \sum_{c \in V} {}^1T_{a,k} Y^{1,*}_{a,\gamma} Y^{2,*}_{i,\gamma} Z^*_{\gamma,\zeta} Y^{4,*}_{j,\zeta} {}^2D^{a,i,b,j} {}^2T_{c,l,b,j} V_{k,i,l,c} \quad (9030)$$

Raw expression

$${}^2R^3_{b,\zeta} \leftarrow - \sum_{\gamma \in A} \sum_{i \in O} \sum_{j \in O} \sum_{k \in O} \sum_{l \in O} \sum_{a \in V} \sum_{c \in V} {}^1T_{a,k} Y^{1,*}_{a,\gamma} Y^{2,*}_{i,\gamma} Z^*_{\gamma,\zeta} Y^{4,*}_{j,\zeta} {}^2D^{a,i,b,j} {}^2T_{b,j,c,l} V_{k,i,l,c} \quad (9018)$$

Factorized expression

$$\tau^0_{\gamma,\delta,w} = \sum_{i \in O} {}^2D^4_{i,w} Y^2_{i,\gamma} Y^{4,*}_{i,\delta} \quad (3r_D r_T^2 N_o) \quad (9019)$$

$$\tau^1_{\alpha,i} = \sum_{a \in V} {}^1T_{a,i} W^2_{a,\alpha} \quad (2r_V N_o N_v) \quad (9020)$$

$$\tau^2_{\gamma,\alpha,w} = \sum_{i \in O} {}^2D^2_{i,w} Y^{2,*}_{i,\gamma} \tau^1_{\alpha,i} \quad (3r_D r_T r_V N_o) \quad (9021)$$

$$\tau^3_{\gamma,\alpha,w} = \sum_{a \in V} {}^2D^1_{a,w} W^1_{a,\alpha} Y^{1,*}_{a,\gamma} \quad (3r_D r_T r_V N_v) \quad (9022)$$

$$\tau^4_{\gamma,\alpha} = \sum_{a \in V} W^4_{a,\alpha} Y^3_{a,\gamma} \quad (2r_T r_V N_v) \quad (9023)$$

$$\tau^5_{\gamma,\alpha} = \sum_{i \in O} W^3_{i,\alpha} Y^4_{i,\gamma} \quad (2r_T r_V N_o) \quad (9024)$$

$$\tau^6_{\gamma,\alpha} = \sum_{\beta \in B} X_{\alpha,\beta} \tau^4_{\gamma,\beta} \tau^5_{\gamma,\beta} \quad (3r_T r_V^2) \quad (9025)$$

$$\tau^7_{\gamma,\alpha} = \sum_{\delta \in A} Z_{\gamma,\delta} \tau^6_{\delta,\alpha} \quad (2r_T^2 r_V) \quad (9026)$$

$$\tau^8_{\gamma,\delta,w} = \sum_{\alpha \in B} \tau^7_{\gamma,\alpha} \tau^2_{\delta,\alpha,w} \tau^3_{\delta,\alpha,w} \quad (3r_D r_T^2 r_V) \quad (9027)$$

$$\tau^9_{\gamma,\delta,w} = \sum_{\epsilon \in A} Z^*_{\epsilon,\delta} \tau^8_{\gamma,\epsilon,w} \quad (2r_D r_T^3) \quad (9028)$$

$${}^2R^3_{a,\gamma} \leftarrow \sum_{\delta \in A} \sum_{w \in D} {}^2D^3_{a,w} Y^1_{a,\delta} \tau^0_{\delta,\gamma,w} \tau^9_{\delta,\gamma,w} \quad (4r_D r_T^2 N_v) \quad (9029)$$

Factorized expression

$$\tau^0_{\gamma,\delta,w} = \sum_{i \in O} {}^2D^4_{i,w} Y^4_{i,\gamma} Y^{4,*}_{i,\delta} \quad (3r_D r_T^2 N_o) \quad (9031)$$

$$\tau^1_{\alpha,i} = \sum_{a \in V} {}^1T_{a,i} W^2_{a,\alpha} \quad (2r_V N_o N_v) \quad (9032)$$

$$\tau^2_{\gamma,\alpha,w} = \sum_{i \in O} {}^2D^2_{i,w} Y^{2,*}_{i,\gamma} \tau^1_{\alpha,i} \quad (3r_D r_T r_V N_o) \quad (9033)$$

$$\tau^3_{\gamma,\alpha,w} = \sum_{a \in V} {}^2D^1_{a,w} W^1_{a,\alpha} Y^{1,*}_{a,\gamma} \quad (3r_D r_T r_V N_v) \quad (9034)$$

$$\tau^4_{\gamma,\alpha} = \sum_{a \in V} W^4_{a,\alpha} Y^1_{a,\gamma} \quad (2r_T r_V N_v) \quad (9035)$$

$$\tau^5_{\gamma,\alpha} = \sum_{i \in O} W^3_{i,\alpha} Y^2_{i,\gamma} \quad (2r_T r_V N_o) \quad (9036)$$

$$\tau^6_{\gamma,\alpha} = \sum_{\beta \in B} X_{\alpha,\beta} \tau^4_{\gamma,\beta} \tau^5_{\gamma,\beta} \quad (3r_T r_V^2) \quad (9037)$$

$$\tau^7_{\gamma,\alpha} = \sum_{\delta \in A} Z_{\delta,\gamma} \tau^6_{\delta,\alpha} \quad (2r_T^2 r_V) \quad (9038)$$

$$\tau^8_{\gamma,\delta,w} = \sum_{\alpha \in B} \tau^7_{\gamma,\alpha} \tau^2_{\delta,\alpha,w} \tau^3_{\delta,\alpha,w} \quad (3r_D r_T^2 r_V) \quad (9039)$$

$$\tau^9_{\gamma,\delta,w} = \sum_{\epsilon \in A} Z^*_{\epsilon,\delta} \tau^8_{\gamma,\epsilon,w} \quad (2r_D r_T^3) \quad (9040)$$

$${}^2R^3_{a,\gamma} \leftarrow \sum_{\delta \in A} \sum_{w \in D} {}^2D^3_{a,w} Y^3_{a,\delta} \tau^0_{\delta,\gamma,w} \tau^9_{\delta,\gamma,w} \quad (4r_D r_T^2 N_v) \quad (9041)$$

Raw expression

$${}^2R^3_{b,\zeta} \leftarrow - \sum_{\gamma \in A} \sum_{i \in O} \sum_{j \in O} \sum_{k \in O} \sum_{l \in O} \sum_{a \in V} \sum_{c \in V} {}^1T_{b,k} Y^{1,*}_{a,\gamma} Y^{2,*}_{i,\gamma} Z^*_{\gamma,\zeta} Y^{4,*}_{j,\zeta} {}^2D^{a,i,b,j} {}^2T_{a,i,c,l} V_{l,c,k,j} \quad (9042)$$

Factorized expression

$$\tau^0_{\alpha,i} = \sum_{a \in V} {}^1T_{a,i} W^2_{a,\alpha} \quad (2r_V N_o N_v) \quad (9043)$$

$$\tau^1_{\gamma,\alpha,w} = \sum_{i \in O} {}^2D^4_{i,w} Y^{4,*}_{i,\gamma} \tau^0_{\alpha,i} \quad (3r_D r_T r_V N_o) \quad (9044)$$

$$\tau^2_{\gamma,\alpha} = \sum_{a \in V} W^4_{a,\alpha} Y^3_{a,\gamma} \quad (2r_T r_V N_v) \quad (9045)$$

$$\tau^3_{\gamma,\alpha} = \sum_{i \in O} W^3_{i,\alpha} Y^4_{i,\gamma} \quad (2r_T r_V N_o) \quad (9046)$$

$$\tau^4_{\gamma,\alpha} = \sum_{\beta \in B} X_{\alpha,\beta} \tau^2_{\gamma,\beta} \tau^3_{\gamma,\beta} \quad (3r_T r_V^2) \quad (9047)$$

$$\tau^5_{\gamma,\alpha} = \sum_{\delta \in A} Z_{\gamma,\delta} \tau^4_{\delta,\alpha} \quad (2r_T^2 r_V) \quad (9048)$$

$$\tau^6_{\gamma,\delta,w} = \sum_{a \in V} {}^2D^1_{a,w} Y^1_{a,\gamma} Y^{1,*}_{a,\delta} \quad (3r_D r_T^2 N_v) \quad (9049)$$

$$\tau^7_{\gamma,\delta,w} = \sum_{i \in O} {}^2D^2_{i,w} Y^2_{i,\gamma} Y^{2,*}_{i,\delta} \quad (3r_D r_T^2 N_o) \quad (9050)$$

$$\tau^8_{\gamma,\delta,w} = \sum_{\epsilon \in A} Z^*_{\epsilon,\delta} \tau^6_{\gamma,\epsilon,w} \tau^7_{\gamma,\epsilon,w} \quad (3r_D r_T^3) \quad (9051)$$

$$\tau^9_{\gamma,\alpha,w} = \sum_{\delta \in A} \tau^5_{\delta,\alpha} \tau^8_{\delta,\gamma,w} \quad (2r_D r_T^2 r_V) \quad (9052)$$

$$\tau^{10}_{\gamma,w,a} = \sum_{\alpha \in B} W^1_{a,\alpha} \tau^1_{\gamma,\alpha,w} \tau^9_{\gamma,\alpha,w} \quad (3r_D r_T r_V N_v) \quad (9053)$$

$${}^2R^3_{a,\gamma} \leftarrow \sum_{w \in D} {}^2D^3_{a,w} \tau^{10}_{\gamma,w,a} \quad (2r_D r_T N_v) \quad (9054)$$

Raw expression

$${}^2R^3_{b,\zeta} \leftarrow - \sum_{\gamma \in A} \sum_{i \in O} \sum_{j \in O} \sum_{k \in O} \sum_{l \in O} \sum_{a \in V} \sum_{c \in V} {}^1T_{b,k} Y^{1,*}_{a,\gamma} Y^{2,*}_{i,\gamma} Z^*_{\gamma,\zeta} Y^{4,*}_{j,\zeta} {}^2D^{a,i,b,j} {}^2T_{c,l,a,i} V_{l,c,k,j} \quad (9055)$$

Factorized expression

$$\tau^0_{\alpha,i} = \sum_{a \in V} {}^1T_{a,i} W^2_{a,\alpha} \quad (2r_V N_o N_v) \quad (9056)$$

$$\tau^1_{\gamma,\alpha,w} = \sum_{i \in O} {}^2D^4_{i,w} Y^{4,*}_{i,\gamma} \tau^0_{\alpha,i} \quad (3r_D r_T r_V N_o) \quad (9057)$$

$$\tau^2_{\gamma,\delta,w} = \sum_{a \in V} {}^2D^1_{a,w} Y^3_{a,\gamma} Y^{1,*}_{a,\delta} \quad (3r_D r_T^2 N_v) \quad (9058)$$

$$\tau^3_{\gamma,\delta,w} = \sum_{i \in O} {}^2D^2_{i,w} Y^4_{i,\gamma} Y^{2,*}_{i,\delta} \quad (3r_D r_T^2 N_o) \quad (9059)$$

$$\tau^4_{\gamma,\delta,w} = \sum_{\epsilon \in A} Z^*_{\epsilon,\delta} \tau^2_{\gamma,\epsilon,w} \tau^3_{\gamma,\epsilon,w} \quad (3r_D r_T^3) \quad (9060)$$

$$\tau^5_{\gamma,\alpha} = \sum_{a \in V} W^4_{a,\alpha} Y^1_{a,\gamma} \quad (2r_T r_V N_v) \quad (9061)$$

$$\tau^6_{\gamma,\alpha} = \sum_{i \in O} W^3_{i,\alpha} Y^2_{i,\gamma} \quad (2r_T r_V N_o) \quad (9062)$$

$$\tau^7_{\gamma,\alpha} = \sum_{\beta \in B} X_{\alpha,\beta} \tau^5_{\gamma,\beta} \tau^6_{\gamma,\beta} \quad (3r_T r_V^2) \quad (9063)$$

$$\tau^8_{\gamma,\alpha} = \sum_{\delta \in A} Z_{\delta,\gamma} \tau^7_{\delta,\alpha} \quad (2r_T^2 r_V) \quad (9064)$$

$$\tau^9_{\gamma,\alpha,w} = \sum_{\delta \in A} \tau^8_{\delta,\alpha} \tau^4_{\delta,\gamma,w} \quad (2r_D r_T^2 r_V) \quad (9065)$$

$$\tau^{10}_{\gamma,w,a} = \sum_{\alpha \in B} W^1_{a,\alpha} \tau^1_{\gamma,\alpha,w} \tau^9_{\gamma,\alpha,w} \quad (3r_D r_T r_V N_v) \quad (9066)$$

$${}^2R^3_{a,\gamma} \leftarrow \sum_{w \in D} {}^2D^3_{a,w} \tau^{10}_{\gamma,w,a} \quad (2r_D r_T N_v) \quad (9067)$$

Raw expression

$${}^2R^3_{b,\zeta} \leftarrow - \sum_{\gamma \in A} \sum_{i \in O} \sum_{j \in O} \sum_{k \in O} \sum_{l \in O} \sum_{a \in V} \sum_{c \in V} {}^1T_{c,k} Y^{1,*}_{a,\gamma} Y^{2,*}_{i,\gamma} Z^*_{\gamma,\zeta} Y^{4,*}_{j,\zeta} {}^2D^{a,i,b,j} {}^2T_{a,i,b,l} V_{k,c,l,j} \quad (9068)$$

Factorized expression

$$\tau^0_{\gamma,\delta,w} = \sum_{i \in O} {}^2D^4_{i,w} Y^2_{i,\gamma} Y^{4,*}_{i,\delta} \quad (3r_D r_T^2 N_o) \quad (9069)$$

$$\tau^1_{\gamma,\delta,w} = \sum_{i \in O} {}^2D^2_{i,w} Y^2_{i,\gamma} Y^{2,*}_{i,\delta} \quad (3r_D r_T^2 N_o) \quad (9082)$$

$$\tau^1_{\gamma,\delta,w} = \sum_{i \in O} {}^2D^2_{i,w} Y^4_{i,\gamma} Y^{2,*}_{i,\delta} \quad (3r_D r_T^2 N_o) \quad (9070)$$

$$\tau^2_{\alpha,i} = \sum_{a \in V} {}^1T_{a,i} W^4_{a,\alpha} \quad (2r_V N_o N_v) \quad (9083)$$

$$\tau^2_{\alpha,i} = \sum_{a \in V} {}^1T_{a,i} W^4_{a,\alpha} \quad (2r_V N_o N_v) \quad (9071)$$

$$\tau^3_{\alpha} = \sum_{i \in O} W^3_{i,\alpha} \tau^2_{\alpha,i} \quad (2r_V N_o) \quad (9084)$$

$$\tau^3_{\alpha} = \sum_{i \in O} W^3_{i,\alpha} \tau^2_{\alpha,i} \quad (2r_V N_o) \quad (9072)$$

$$\tau^4_{\alpha} = \sum_{\beta \in B} \tau^3_{\beta} X_{\alpha,\beta} \quad (2r_V^2) \quad (9085)$$

$$\tau^4_{\alpha} = \sum_{\beta \in B} \tau^3_{\beta} X_{\alpha,\beta} \quad (2r_V^2) \quad (9073)$$

$$\tau^5_{a,b} = \sum_{\alpha \in B} \tau^4_{\alpha} W^1_{a,\alpha} W^2_{b,\alpha} \quad (3r_V N_v^2) \quad (9086)$$

$$\tau^5_{a,b} = \sum_{\alpha \in B} \tau^4_{\alpha} W^1_{a,\alpha} W^2_{b,\alpha} \quad (3r_V N_v^2) \quad (9074)$$

$$\tau^6_{\gamma,a} = \sum_{b \in V} Y^1_{b,\gamma} \tau^5_{a,b} \quad (2r_T N_v^2) \quad (9087)$$

$$\tau^6_{\gamma,a} = \sum_{b \in V} Y^3_{b,\gamma} \tau^5_{a,b} \quad (2r_T N_v^2) \quad (9075)$$

$$\tau^7_{\gamma,\delta,w} = \sum_{a \in V} {}^2D^1_{a,w} Y^{1,*}_{a,\delta} \tau^6_{\gamma,a} \quad (3r_D r_T^2 N_v) \quad (9088)$$

$$\tau^7_{\gamma,\delta,w} = \sum_{a \in V} {}^2D^1_{a,w} Y^{1,*}_{a,\delta} \tau^6_{\gamma,a} \quad (3r_D r_T^2 N_v) \quad (9076)$$

$$\tau^8_{\gamma,\delta,w} = \sum_{\epsilon \in A} Z^*_{\epsilon,\delta} \tau^1_{\gamma,\epsilon,w} \tau^7_{\gamma,\epsilon,w} \quad (3r_D r_T^3) \quad (9089)$$

$$\tau^8_{\gamma,\delta,w} = \sum_{\epsilon \in A} Z^*_{\epsilon,\delta} \tau^1_{\gamma,\epsilon,w} \tau^7_{\gamma,\epsilon,w} \quad (3r_D r_T^3) \quad (9077)$$

$$\tau^9_{\gamma,\delta,w} = \sum_{\epsilon \in A} Z_{\epsilon,\gamma} \tau^8_{\epsilon,\delta,w} \quad (2r_D r_T^3) \quad (9090)$$

$$\tau^9_{\gamma,\delta,w} = \sum_{\epsilon \in A} Z_{\gamma,\epsilon} \tau^8_{\epsilon,\delta,w} \quad (2r_D r_T^3) \quad (9078)$$

$${}^2R^3_{a,\gamma} \leftarrow \sum_{\delta \in A} \sum_{w \in D} {}^2D^3_{a,w} Y^3_{a,\delta} \tau^0_{\delta,\gamma,w} \tau^9_{\delta,\gamma,w} \quad (4r_D r_T^2 N_v) \quad (9091)$$

$${}^2R^3_{a,\gamma} \leftarrow \sum_{\delta \in A} \sum_{w \in D} {}^2D^3_{a,w} Y^1_{a,\delta} \tau^0_{\delta,\gamma,w} \tau^9_{\delta,\gamma,w} \quad (4r_D r_T^2 N_v) \quad (9079)$$

Raw expression

$${}^2R^3_{b,\zeta} \leftarrow - \sum_{\gamma \in A} \sum_{i \in O} \sum_{j \in O} \sum_{k \in O} \sum_{l \in O} \sum_{a \in V} \sum_{c \in V} {}^1T_{c,k} Y^{1,*}_{a,\gamma} Y^{2,*}_{i,\gamma} Z^*_{\gamma,\zeta} Y^{4,*}_{j,\zeta} {}^2D^{a,i,b,j} {}^2T_{b,j,a,l} V_{l,i,k,c} \quad (9092)$$

Raw expression

$${}^2R^3_{b,\zeta} \leftarrow - \sum_{\gamma \in A} \sum_{i \in O} \sum_{j \in O} \sum_{k \in O} \sum_{l \in O} \sum_{a \in V} \sum_{c \in V} {}^1T_{c,k} Y^{1,*}_{a,\gamma} Y^{2,*}_{i,\gamma} Z^*_{\gamma,\zeta} Y^{4,*}_{j,\zeta} {}^2D^{a,i,b,j} {}^2T_{a,l,b,j} V_{l,i,k,c} \quad (9080)$$

Factorized expression

Factorized expression

$$\tau^0_{\alpha,i} = \sum_{a \in V} {}^1T_{a,i} W^4_{a,\alpha} \quad (2r_V N_o N_v) \quad (9093)$$

$$\tau^0_{\gamma,\delta,w} = \sum_{i \in O} {}^2D^4_{i,w} Y^4_{i,\gamma} Y^{4,*}_{i,\delta} \quad (3r_D r_T^2 N_o) \quad (9081)$$

$$\tau^1_{\alpha} = \sum_{i \in O} W^3_{i,\alpha} \tau^0_{\alpha,i} \quad (2r_V N_o) \quad (9094)$$

$$\tau^2_\alpha = \sum_{\beta \in B} \tau^1_\beta X_{\alpha,\beta} \quad (2r_V^2) \quad (9095)$$

$$\tau^3_{a,b} = \sum_{\alpha \in B} \tau^2_\alpha W^1_{a,\alpha} W^2_{b,\alpha} \quad (3r_V N_v^2) \quad (9096)$$

$$\tau^4_{\gamma,a} = \sum_{b \in V} Y^3_{b,\gamma} \tau^3_{a,b} \quad (2r_T N_v^2) \quad (9097)$$

$$\tau^5_{\gamma,\delta,w} = \sum_{i \in O} {}^2D^4_{i,w} Y^4_{i,\gamma} Y^{4,*}_{i,\delta} \quad (3r_D r_T^2 N_o) \quad (9098)$$

$$\tau^6_{\gamma,\delta,w} = \sum_{a \in V} {}^2D^1_{a,w} Y^1_{a,\gamma} Y^{1,*}_{a,\delta} \quad (3r_D r_T^2 N_v) \quad (9099)$$

$$\tau^7_{\gamma,\delta,w} = \sum_{i \in O} {}^2D^2_{i,w} Y^2_{i,\gamma} Y^{2,*}_{i,\delta} \quad (3r_D r_T^2 N_o) \quad (9100)$$

$$\tau^8_{\gamma,\delta,w} = \sum_{\epsilon \in A} Z^*_{\epsilon,\delta} \tau^6_{\gamma,\epsilon,w} \tau^7_{\gamma,\epsilon,w} \quad (3r_D r_T^3) \quad (9101)$$

$$\tau^9_{\gamma,\delta,w} = \sum_{\epsilon \in A} Z_{\epsilon,\gamma} \tau^8_{\epsilon,\delta,w} \quad (2r_D r_T^3) \quad (9102)$$

$${}^2R^3_{a,\gamma} \leftarrow \sum_{\delta \in A} \sum_{w \in D} {}^2D^3_{a,w} \tau^4_{\delta,a} \tau^5_{\delta,\gamma,w} \tau^9_{\delta,\gamma,w} \quad (4r_D r_T^2 N_v) \quad (9103)$$

Raw expression

$${}^2R^3_{b,\zeta} \leftarrow - \sum_{\gamma \in A} \sum_{i \in O} \sum_{j \in O} \sum_{k \in O} \sum_{l \in O} \sum_{a \in V} \sum_{c \in V} {}^1T_{c,k} Y^{1,*}_{a,\gamma} Y^{2,*}_{i,\gamma} Z^*_{\gamma,\zeta} Y^{4,*}_{j,\zeta} {}^2D^{a,i,b,j} {}^2T_{b,l,a,i} V_{k,c,l,j} \quad (9104)$$

Factorized expression

$$\tau^0_{\alpha,i} = \sum_{a \in V} {}^1T_{a,i} W^4_{a,\alpha} \quad (2r_V N_o N_v) \quad (9105)$$

$$\tau^1_\alpha = \sum_{i \in O} W^3_{i,\alpha} \tau^0_{\alpha,i} \quad (2r_V N_o) \quad (9106)$$

$$\tau^2_\alpha = \sum_{\beta \in B} \tau^1_\beta X_{\alpha,\beta} \quad (2r_V^2) \quad (9107)$$

$$\tau^3_{a,b} = \sum_{\alpha \in B} \tau^2_\alpha W^1_{a,\alpha} W^2_{b,\alpha} \quad (3r_V N_v^2) \quad (9108)$$

$$\tau^4_{\gamma,a} = \sum_{b \in V} Y^1_{b,\gamma} \tau^3_{a,b} \quad (2r_T N_v^2) \quad (9109)$$

$$\tau^5_{\gamma,\delta,w} = \sum_{i \in O} {}^2D^4_{i,w} Y^2_{i,\gamma} Y^{4,*}_{i,\delta} \quad (3r_D r_T^2 N_o) \quad (9110)$$

$$\tau^6_{\gamma,\delta,w} = \sum_{a \in V} {}^2D^1_{a,w} Y^3_{a,\gamma} Y^{1,*}_{a,\delta} \quad (3r_D r_T^2 N_v) \quad (9111)$$

$$\tau^7_{\gamma,\delta,w} = \sum_{i \in O} {}^2D^2_{i,w} Y^4_{i,\gamma} Y^{2,*}_{i,\delta} \quad (3r_D r_T^2 N_o) \quad (9112)$$

$$\tau^8_{\gamma,\delta,w} = \sum_{\epsilon \in A} Z^*_{\epsilon,\delta} \tau^6_{\gamma,\epsilon,w} \tau^7_{\gamma,\epsilon,w} \quad (3r_D r_T^3) \quad (9113)$$

$$\tau^9_{\gamma,\delta,w} = \sum_{\epsilon \in A} Z_{\gamma,\epsilon} \tau^8_{\epsilon,\delta,w} \quad (2r_D r_T^3) \quad (9114)$$

$${}^2R^3_{a,\gamma} \leftarrow \sum_{\delta \in A} \sum_{w \in D} {}^2D^3_{a,w} \tau^4_{\delta,a} \tau^5_{\delta,\gamma,w} \tau^9_{\delta,\gamma,w} \quad (4r_D r_T^2 N_v) \quad (9115)$$

Raw expression

$${}^2R^3_{b,\zeta} \leftarrow \sum_{\gamma \in A} \sum_{i \in O} \sum_{j \in O} \sum_{k \in O} \sum_{a \in V} \sum_{c \in V} \sum_{d \in V} {}^1T_{c,i} Y^{1,*}_{a,\gamma} Y^{2,*}_{i,\gamma} Z^*_{\gamma,\zeta} Y^{4,*}_{j,\zeta} {}^2D^{a,i,b,j} {}^2T_{b,j,d,k} V_{a,c,k,d} \quad (9116)$$

Factorized expression

$$\tau^0_{\gamma,\alpha} = \sum_{a \in V} W^2_{a,\alpha} Y^1_{a,\gamma} \quad (2r_T r_V N_v) \quad (9117)$$

$$\tau^1_{\gamma,\alpha,i} = \sum_{\delta \in A} Y^2_{i,\delta} Z_{\delta,\gamma} \tau^0_{\delta,\alpha} \quad (3r_T^2 r_V N_o) \quad (9118)$$

$$\tau^2_{\gamma,w,i} = \sum_{a \in V} {}^2D^1_{a,w} {}^1T_{a,i} Y^{1,*}_{a,\gamma} \quad (3r_D r_T N_o N_v) \quad (9119)$$

$$\tau^3_{\gamma,w,i,j} = \sum_{\delta \in A} Y^{2,*}_{j,\delta} Z^*_{\delta,\gamma} \tau^2_{\delta,w,i} \quad (3r_D r_T^2 N_o^2) \quad (9120)$$

$$\tau_{\gamma,\delta,w,i}^4 = \sum_{j \in O} {}^2D_{j,w}^2 Y_{j,\gamma}^4 \tau_{\delta,w,i,j}^3 \quad (3r_D r_T^2 N_o^2) \quad (9121)$$

$$\tau_{\gamma,\delta,w,i}^4 = \sum_{j \in O} {}^2D_{j,w}^2 Y_{j,\gamma}^2 \tau_{\delta,w,i,j}^3 \quad (3r_D r_T^2 N_o^2) \quad (9134)$$

$$\tau_{\gamma,\alpha}^5 = \sum_{a \in V} W_{a,\alpha}^4 Y_{a,\gamma}^3 \quad (2r_T r_V N_v) \quad (9122)$$

$$\tau_{\gamma,\alpha}^5 = \sum_{a \in V} W_{a,\alpha}^4 Y_{a,\gamma}^1 \quad (2r_T r_V N_v) \quad (9135)$$

$$\tau_{\gamma,\alpha,i}^6 = \sum_{\beta \in B} X_{\alpha,\beta} W_{i,\beta}^3 \tau_{\gamma,\beta}^5 \quad (3r_T r_V^2 N_o) \quad (9123)$$

$$\tau_{\gamma,\alpha,i}^6 = \sum_{\beta \in B} X_{\alpha,\beta} W_{i,\beta}^3 \tau_{\gamma,\beta}^5 \quad (3r_T r_V^2 N_o) \quad (9136)$$

$$\tau_{\gamma,\delta,\alpha,w}^7 = \sum_{i \in O} \tau_{\gamma,\alpha,i}^6 \tau_{\gamma,\delta,w,i}^4 \quad (2r_D r_T^2 r_V N_o) \quad (9124)$$

$$\tau_{\gamma,\delta,\alpha,w}^7 = \sum_{i \in O} \tau_{\gamma,\alpha,i}^6 \tau_{\gamma,\delta,w,i}^4 \quad (2r_D r_T^2 r_V N_o) \quad (9137)$$

$$\tau_{\gamma,\alpha,w,i}^8 = \sum_{\delta \in A} \tau_{\delta,\alpha,i}^1 \tau_{\delta,\gamma,\alpha,w}^7 \quad (2r_D r_T^2 r_V N_o) \quad (9125)$$

$$\tau_{\gamma,\alpha,w,i}^8 = \sum_{\delta \in A} \tau_{\delta,\alpha,i}^1 \tau_{\delta,\gamma,\alpha,w}^7 \quad (2r_D r_T^2 r_V N_o) \quad (9138)$$

$$\tau_{\gamma,\alpha,w}^9 = \sum_{i \in O} {}^2D_{i,w}^4 Y_{i,\gamma}^{4,*} \tau_{\gamma,\alpha,w,i}^8 \quad (3r_D r_T r_V N_o) \quad (9126)$$

$$\tau_{\gamma,\alpha,w}^9 = \sum_{i \in O} {}^2D_{i,w}^4 Y_{i,\gamma}^{4,*} \tau_{\gamma,\alpha,w,i}^8 \quad (3r_D r_T r_V N_o) \quad (9139)$$

$$\tau_{\gamma,w,a}^{10} = \sum_{\alpha \in B} W_{a,\alpha}^1 \tau_{\gamma,\alpha,w}^9 \quad (2r_D r_T r_V N_v) \quad (9127)$$

$$\tau_{\gamma,w,a}^{10} = \sum_{\alpha \in B} W_{a,\alpha}^1 \tau_{\gamma,\alpha,w}^9 \quad (2r_D r_T r_V N_v) \quad (9140)$$

$${}^2R_{a,\gamma}^3 \leftarrow - \sum_{w \in D} \frac{1}{2} {}^2D_{a,w}^3 \tau_{\gamma,w,a}^{10} \quad (2r_D r_T N_v) \quad (9128)$$

$${}^2R_{a,\gamma}^3 \leftarrow - \sum_{w \in D} \frac{1}{2} {}^2D_{a,w}^3 \tau_{\gamma,w,a}^{10} \quad (2r_D r_T N_v) \quad (9141)$$

Raw expression

$${}^2R_{b,\zeta}^3 \leftarrow \sum_{\gamma \in A} \sum_{i \in O} \sum_{j \in O} \sum_{k \in O} \sum_{a \in V} \sum_{c \in V} \sum_{d \in V} {}^1T_{c,i} Y_{a,\gamma}^{1,*} Y_{i,\gamma}^{2,*} Z_{\gamma,\zeta}^* Y_{j,\zeta}^{4,*} {}^2D_{a,i,b,j} {}^2T_{d,k,b,j} V_{a,c,k,d} \quad (9129)$$

Raw expression

$${}^2R_{b,\zeta}^3 \leftarrow \sum_{\gamma \in A} \sum_{i \in O} \sum_{j \in O} \sum_{k \in O} \sum_{a \in V} \sum_{c \in V} \sum_{d \in V} {}^1T_{c,j} Y_{a,\gamma}^{1,*} Y_{i,\gamma}^{2,*} Z_{\gamma,\zeta}^* Y_{j,\zeta}^{4,*} {}^2D_{a,i,b,j} {}^2T_{a,i,d,k} V_{b,c,k,d} \quad (9142)$$

Factorized expression

$$\tau_{\gamma,\alpha}^0 = \sum_{a \in V} W_{a,\alpha}^2 Y_{a,\gamma}^3 \quad (2r_T r_V N_v) \quad (9130)$$

$$\tau_{\gamma,\alpha,w}^0 = \sum_{a \in V} {}^2D_{a,w}^1 W_{a,\alpha}^1 Y_{a,\gamma}^{1,*} \quad (3r_D r_T r_V N_v) \quad (9143)$$

$$\tau_{\gamma,\alpha,i}^1 = \sum_{\delta \in A} Z_{\gamma,\delta} Y_{i,\delta}^4 \tau_{\delta,\alpha}^0 \quad (3r_T^2 r_V N_o) \quad (9131)$$

$$\tau_{\gamma,\alpha}^1 = \sum_{a \in V} W_{a,\alpha}^2 Y_{a,\gamma}^1 \quad (2r_T r_V N_v) \quad (9144)$$

$$\tau_{\gamma,w,i}^2 = \sum_{a \in V} {}^2D_{a,w}^1 T_{a,i} {}^1Y_{a,\gamma}^{1,*} \quad (3r_D r_T N_o N_v) \quad (9132)$$

$$\tau_{\gamma,\alpha,i}^2 = \sum_{\delta \in A} Y_{i,\delta}^2 Z_{\delta,\gamma} \tau_{\delta,\alpha}^1 \quad (3r_T^2 r_V N_o) \quad (9145)$$

$$\tau_{\gamma,w,i,j}^3 = \sum_{\delta \in A} Y_{j,\delta}^{2,*} Z_{\delta,\gamma}^* \tau_{\delta,w,i}^2 \quad (3r_D r_T^2 N_o^2) \quad (9133)$$

$$\tau_{\gamma,\delta,\alpha,w}^3 = \sum_{i \in O} {}^2D_{i,w}^2 Y_{i,\delta}^{2,*} \tau_{\delta,\alpha,w}^0 \tau_{\gamma,\alpha,i}^2 \quad (4r_D r_T^2 r_V N_o) \quad (9146)$$

$$\tau^4_{\gamma,\alpha} = \sum_{a \in V} W^4_{a,\alpha} Y^3_{a,\gamma} \quad (2r_T r_V N_v) \quad (9147)$$

$$\tau^5_{\gamma,\alpha,i} = \sum_{\beta \in B} X_{\alpha,\beta} W^3_{i,\beta} \tau^4_{\gamma,\beta} \quad (3r_T r_V^2 N_o) \quad (9148)$$

$$\tau^6_{\gamma,\delta,w,i} = \sum_{\alpha \in B} \tau^5_{\gamma,\alpha,i} \tau^3_{\gamma,\delta,\alpha,w} \quad (2r_D r_T^2 r_V N_o) \quad (9149)$$

$$\tau^7_{\gamma,w,i,j} = \sum_{\delta \in A} {}^2D^4_{i,w} Y^4_{i,\delta} \tau^6_{\delta,\gamma,w,j} \quad (3r_D r_T^2 N_o^2) \quad (9150)$$

$$\tau^8_{\gamma,w,i} = \sum_{\delta \in A} \sum_{j \in O} Z^*_{\delta,\gamma} Y^{4,*}_{j,\gamma} \tau^7_{\delta,w,j,i} \quad (3r_D r_T^2 N_o^2) \quad (9151)$$

$${}^2R^3_{a,\gamma} \leftarrow - \sum_{w \in D} \sum_{i \in O} \frac{1}{2} {}^2D^3_{a,w} {}^1T_{a,i} \tau^8_{\gamma,w,i} \quad (3r_D r_T N_o N_v) \quad (9152)$$

Raw expression

$${}^2R^3_{b,\zeta} \leftarrow \sum_{\gamma \in A} \sum_{i \in O} \sum_{j \in O} \sum_{k \in O} \sum_{a \in V} \sum_{c \in V} \sum_{d \in V} {}^1T_{c,j} Y^{1,*}_{a,\gamma} Y^{2,*}_{i,\gamma} Z^*_{\gamma,\zeta} Y^{4,*}_{j,\zeta} {}^2D^{a,i,b,j} {}^2T_{d,k,a,i} V_{b,c,k,d} \quad (9153)$$

Factorized expression

$$\tau^0_{\gamma,\alpha,w} = \sum_{a \in V} {}^2D^1_{a,w} W^1_{a,\alpha} Y^{1,*}_{a,\gamma} \quad (3r_D r_T r_V N_v) \quad (9154)$$

$$\tau^1_{\gamma,\alpha} = \sum_{a \in V} W^2_{a,\alpha} Y^3_{a,\gamma} \quad (2r_T r_V N_v) \quad (9155)$$

$$\tau^2_{\gamma,\alpha,i} = \sum_{\delta \in A} Z_{\gamma,\delta} Y^4_{i,\delta} \tau^1_{\delta,\alpha} \quad (3r_T^2 r_V N_o) \quad (9156)$$

$$\tau^3_{\gamma,\delta,\alpha,w} = \sum_{i \in O} {}^2D^2_{i,w} Y^{2,*}_{i,\delta} \tau^0_{\delta,\alpha,w} \tau^2_{\gamma,\alpha,i} \quad (4r_D r_T^2 r_V N_o) \quad (9157)$$

$$\tau^4_{\gamma,\alpha} = \sum_{a \in V} W^4_{a,\alpha} Y^1_{a,\gamma} \quad (2r_T r_V N_v) \quad (9158)$$

$$\tau^5_{\gamma,\alpha,i} = \sum_{\beta \in B} X_{\alpha,\beta} W^3_{i,\beta} \tau^4_{\gamma,\beta} \quad (3r_T r_V^2 N_o) \quad (9159)$$

$$\tau^6_{\gamma,\delta,w,i} = \sum_{\alpha \in B} \tau^5_{\gamma,\alpha,i} \tau^3_{\gamma,\delta,\alpha,w} \quad (2r_D r_T^2 r_V N_o) \quad (9160)$$

$$\tau^7_{\gamma,w,i,j} = \sum_{\delta \in A} {}^2D^4_{i,w} Y^2_{i,\delta} \tau^6_{\delta,\gamma,w,j} \quad (3r_D r_T^2 N_o^2) \quad (9161)$$

$$\tau^8_{\gamma,w,i} = \sum_{\delta \in A} \sum_{j \in O} Z^*_{\delta,\gamma} Y^{4,*}_{j,\gamma} \tau^7_{\delta,w,j,i} \quad (3r_D r_T^2 N_o^2) \quad (9162)$$

$${}^2R^3_{a,\gamma} \leftarrow - \sum_{w \in D} \sum_{i \in O} \frac{1}{2} {}^2D^3_{a,w} {}^1T_{a,i} \tau^8_{\gamma,w,i} \quad (3r_D r_T N_o N_v) \quad (9163)$$

Raw expression

$${}^2R^3_{b,\zeta} \leftarrow \sum_{\gamma \in A} \sum_{i \in O} \sum_{j \in O} \sum_{k \in O} \sum_{a \in V} \sum_{c \in V} \sum_{d \in V} {}^1T_{c,k} Y^{1,*}_{a,\gamma} Y^{2,*}_{i,\gamma} Z^*_{\gamma,\zeta} Y^{4,*}_{j,\zeta} {}^2D^{a,i,b,j} {}^2T_{a,i,d,j} V_{b,d,k,c} \quad (9164)$$

Factorized expression

$$\tau^0_{\gamma,\alpha} = \sum_{i \in O} W^3_{i,\alpha} Y^2_{i,\gamma} \quad (2r_T r_V N_o) \quad (9165)$$

$$\tau^1_{\gamma,\alpha} = \sum_{a \in V} W^4_{a,\alpha} Y^3_{a,\gamma} \quad (2r_T r_V N_v) \quad (9166)$$

$$\tau^2_{\gamma,\alpha,i} = \sum_{\delta \in A} Z_{\gamma,\delta} Y^4_{i,\delta} \tau^1_{\delta,\alpha} \quad (3r_T^2 r_V N_o) \quad (9167)$$

$$\tau^3_{\alpha,i} = \sum_{a \in V} {}^1T_{a,i} W^2_{a,\alpha} \quad (2r_V N_o N_v) \quad (9168)$$

$$\tau^4_{\gamma,\alpha,w} = \sum_{i \in O} {}^2D^2_{i,w} Y^{2,*}_{i,\gamma} \tau^3_{\alpha,i} \quad (3r_D r_T r_V N_o) \quad (9169)$$

$$\tau^5_{\gamma,\alpha,w} = \sum_{a \in V} {}^2D^1_{a,w} W^1_{a,\alpha} Y^{1,*}_{a,\gamma} \quad (3r_D r_T r_V N_v) \quad (9170)$$



$$\tau^6_{\gamma,\alpha,w} = \sum_{\beta \in B} X_{\beta,\alpha} \tau^4_{\gamma,\beta,w} \tau^5_{\gamma,\beta,w} \quad (3r_D r_T r_V^2) \quad (9171)$$

$$\tau^7_{\gamma,\alpha,w} = \sum_{\delta \in A} Z^*_{\delta,\gamma} \tau^6_{\delta,\alpha,w} \quad (2r_D r_T^2 r_V) \quad (9172)$$

$$\tau^8_{\gamma,\delta,w,i} = \sum_{\alpha \in B} \tau^0_{\gamma,\alpha} \tau^2_{\gamma,\alpha,i} \tau^7_{\delta,\alpha,w} \quad (3r_D r_T^2 r_V N_o) \quad (9173)$$

$$\tau^9_{\gamma,\delta,w} = \sum_{i \in O} {}^2D^4_{i,w} Y^{4,*}_{i,\delta} \tau^8_{\gamma,\delta,w,i} \quad (3r_D r_T^2 N_o) \quad (9174)$$

$${}^2R^3_{a,\gamma} \leftarrow - \sum_{\delta \in A} \sum_{w \in D} \frac{1}{2} {}^2D^3_{a,w} Y^1_{a,\delta} \tau^9_{\delta,\gamma,w} \quad (3r_D r_T^2 N_v) \quad (9175)$$

Raw expression

$${}^2R^3_{b,\zeta} \leftarrow \sum_{\gamma \in A} \sum_{i \in O} \sum_{j \in O} \sum_{k \in O} \sum_{a \in V} \sum_{c \in V} \sum_{d \in V} {}^1T_{c,k} Y^{1,*}_{a,\gamma} Y^{2,*}_{i,\gamma} Z^*_{\gamma,\zeta} Y^{4,*}_{j,\zeta} {}^2D^{a,i,b,j} {}^2T_{b,j,d,i} V_{a,d,k,c} \quad (9176)$$

Factorized expression

$$\tau^0_{\gamma,\alpha} = \sum_{a \in V} W^4_{a,\alpha} Y^1_{a,\gamma} \quad (2r_T r_V N_v) \quad (9177)$$

$$\tau^1_{\gamma,\alpha,i} = \sum_{\delta \in A} Y^2_{i,\delta} Z_{\delta,\gamma} \tau^0_{\delta,\alpha} \quad (3r_T^2 r_V N_o) \quad (9178)$$

$$\tau^2_{\gamma,\alpha} = \sum_{i \in O} W^3_{i,\alpha} Y^4_{i,\gamma} \quad (2r_T r_V N_o) \quad (9179)$$

$$\tau^3_{\alpha,i} = \sum_{a \in V} {}^1T_{a,i} W^2_{a,\alpha} \quad (2r_V N_o N_v) \quad (9180)$$

$$\tau^4_{\gamma,\alpha,w} = \sum_{i \in O} {}^2D^2_{i,w} Y^{2,*}_{i,\gamma} \tau^3_{\alpha,i} \quad (3r_D r_T r_V N_o) \quad (9181)$$

$$\tau^5_{\gamma,\alpha,w} = \sum_{a \in V} {}^2D^1_{a,w} W^1_{a,\alpha} Y^{1,*}_{a,\gamma} \quad (3r_D r_T r_V N_v) \quad (9182)$$

$$\tau^6_{\gamma,\alpha,w} = \sum_{\beta \in B} X_{\beta,\alpha} \tau^4_{\gamma,\beta,w} \tau^5_{\gamma,\beta,w} \quad (3r_D r_T r_V^2) \quad (9183)$$

$$\tau^7_{\gamma,\alpha,w} = \sum_{\delta \in A} Z^*_{\delta,\gamma} \tau^6_{\delta,\alpha,w} \quad (2r_D r_T^2 r_V) \quad (9184)$$

$$\tau^8_{\gamma,\delta,w,i} = \sum_{\alpha \in B} \tau^2_{\gamma,\alpha} \tau^1_{\gamma,\alpha,i} \tau^7_{\delta,\alpha,w} \quad (3r_D r_T^2 r_V N_o) \quad (9185)$$

$$\tau^9_{\gamma,\delta,w} = \sum_{i \in O} {}^2D^4_{i,w} Y^{4,*}_{i,\delta} \tau^8_{\gamma,\delta,w,i} \quad (3r_D r_T^2 N_o) \quad (9186)$$

$${}^2R^3_{a,\gamma} \leftarrow - \sum_{\delta \in A} \sum_{w \in D} \frac{1}{2} {}^2D^3_{a,w} Y^3_{a,\delta} \tau^9_{\delta,\gamma,w} \quad (3r_D r_T^2 N_v) \quad (9187)$$

Raw expression

$${}^2R^3_{b,\zeta} \leftarrow \sum_{\gamma \in A} \sum_{i \in O} \sum_{j \in O} \sum_{k \in O} \sum_{a \in V} \sum_{c \in V} \sum_{d \in V} {}^1T_{c,k} Y^{1,*}_{a,\gamma} Y^{2,*}_{i,\gamma} Z^*_{\gamma,\zeta} Y^{4,*}_{j,\zeta} {}^2D^{a,i,b,j} {}^2T_{d,i,b,j} V_{a,d,k,c} \quad (9188)$$

Factorized expression

$$\tau^0_{\gamma,\delta,w} = \sum_{i \in O} {}^2D^4_{i,w} Y^2_{i,\gamma} Y^{4,*}_{i,\delta} \quad (3r_D r_T^2 N_o) \quad (9189)$$

$$\tau^1_{\alpha,i} = \sum_{a \in V} {}^1T_{a,i} W^4_{a,\alpha} \quad (2r_V N_o N_v) \quad (9190)$$

$$\tau^2_{\alpha,i,j} = \sum_{\beta \in B} X_{\alpha,\beta} W^3_{j,\beta} \tau^1_{\beta,i} \quad (3r_V^2 N_o^2) \quad (9191)$$

$$\tau^3_{\gamma,\alpha,i} = \sum_{j \in O} Y^4_{j,\gamma} \tau^2_{\alpha,i,j} \quad (2r_T r_V N_o^2) \quad (9192)$$

$$\tau^4_{\gamma,\alpha} = \sum_{a \in V} W^2_{a,\alpha} Y^3_{a,\gamma} \quad (2r_T r_V N_v) \quad (9193)$$

$$\tau^5_{\gamma,i,a} = \sum_{\alpha \in B} W^1_{a,\alpha} \tau^4_{\gamma,\alpha} \tau^3_{\gamma,\alpha,i} \quad (3r_T r_V N_o N_v) \quad (9194)$$

$$\tau^6_{\gamma,\delta,w} = \sum_{i \in O} \sum_{a \in V} {}^2D^1_{a,w} {}^2D^2_{i,w} Y^{1,*}_{a,\delta} Y^{2,*}_{i,\delta} \tau^5_{\gamma,i,a} \quad (5r_D r_T^2 N_o N_v) \quad (9195)$$

$$\tau_{\gamma,\delta,w}^7 = \sum_{\epsilon \in A} Z_{\epsilon,\delta}^* \tau_{\gamma,\epsilon,w}^6 \quad (2r_D r_T^3) \quad (9196)$$

$${}^2R_{a,\gamma}^3 \leftarrow - \sum_{\delta \in A} \sum_{w \in D} \frac{1}{2} D_{a,w}^3 Y_{a,\delta}^3 \tau_{\delta,\gamma,w}^0 \tau_{\delta,\gamma,w}^8 \quad (4r_D r_T^2 N_v) \quad (9209)$$

$$\tau_{\gamma,\delta,w}^8 = \sum_{\epsilon \in A} Z_{\gamma,\epsilon} \tau_{\epsilon,\delta,w}^7 \quad (2r_D r_T^3) \quad (9197)$$

Raw expression

$${}^2R_{a,\gamma}^3 \leftarrow - \sum_{\delta \in A} \sum_{w \in D} \frac{1}{2} D_{a,w}^3 Y_{a,\delta}^1 \tau_{\delta,\gamma,w}^0 \tau_{\delta,\gamma,w}^8 \quad (4r_D r_T^2 N_v) \quad (9198)$$

$${}^2R_{b,\zeta}^3 \leftarrow - \sum_{\gamma \in A} \sum_{i \in O} \sum_{j \in O} \sum_{k \in O} \sum_{a \in V} \sum_{c \in V} \sum_{d \in V} \frac{1}{2} {}^1T_{a,k} Y_{a,\gamma}^{1,*} Y_{i,\gamma}^{2,*} Z_{\gamma,\zeta}^* Y_{j,\zeta}^{4,*} {}^2D_{a,i,b,j} {}^2T_{c,i,d,j} V_{b,d,k,c} \quad (9210)$$

Raw expression

Factorized expression

$${}^2R_{b,\zeta}^3 \leftarrow \sum_{\gamma \in A} \sum_{i \in O} \sum_{j \in O} \sum_{k \in O} \sum_{a \in V} \sum_{c \in V} \sum_{d \in V} {}^1T_{c,k} Y_{a,\gamma}^{1,*} Y_{i,\gamma}^{2,*} Z_{\gamma,\zeta}^* Y_{j,\zeta}^{4,*} {}^2D_{a,i,b,j} {}^2T_{d,j,a,i} V_{b,d,k,c} \quad (9199)$$

$$\tau_{\gamma,\alpha}^0 = \sum_{a \in V} W_{a,\alpha}^2 Y_{a,\gamma}^3 \quad (2r_T r_V N_v) \quad (9211)$$

$$\tau_{\gamma,\alpha,i}^1 = \sum_{\delta \in A} Z_{\gamma,\delta} Y_{i,\delta}^4 \tau_{\delta,\alpha}^0 \quad (3r_T^2 r_V N_o) \quad (9212)$$

Factorized expression

$$\tau_{\gamma,\delta,w}^0 = \sum_{i \in O} {}^2D_{i,w}^4 Y_{i,\gamma}^4 Y_{i,\delta}^{4,*} \quad (3r_D r_T^2 N_o) \quad (9200)$$

$$\tau_{\gamma,\delta,w}^2 = \sum_{a \in V} {}^2D_{a,w}^1 Y_{a,\gamma}^1 Y_{a,\delta}^{1,*} \quad (3r_D r_T^2 N_v) \quad (9213)$$

$$\tau_{\alpha,i}^1 = \sum_{a \in V} {}^1T_{a,i} W_{a,\alpha}^4 \quad (2r_V N_o N_v) \quad (9201)$$

$$\tau_{\gamma,\delta,w,i}^3 = \sum_{\epsilon \in A} {}^2D_{i,w}^2 Y_{i,\epsilon}^{2,*} Z_{\epsilon,\delta}^* \tau_{\gamma,\epsilon,w}^2 \quad (4r_D r_T^3 N_o) \quad (9214)$$

$$\tau_{\alpha,i,j}^2 = \sum_{\beta \in B} X_{\alpha,\beta} W_{j,\beta}^3 \tau_{\beta,i}^1 \quad (3r_V^2 N_o^2) \quad (9202)$$

$$\tau_{\alpha,i}^4 = \sum_{a \in V} {}^1T_{a,i} W_{a,\alpha}^4 \quad (2r_V N_o N_v) \quad (9215)$$

$$\tau_{\gamma,\alpha,i}^3 = \sum_{j \in O} Y_{j,\gamma}^2 \tau_{\alpha,i,j}^2 \quad (2r_T r_V N_o^2) \quad (9203)$$

$$\tau_{\alpha,i,j}^5 = \sum_{\beta \in B} X_{\alpha,\beta} W_{j,\beta}^3 \tau_{\beta,i}^4 \quad (3r_V^2 N_o^2) \quad (9216)$$

$$\tau_{\gamma,\alpha}^4 = \sum_{a \in V} W_{a,\alpha}^2 Y_{a,\gamma}^1 \quad (2r_T r_V N_v) \quad (9204)$$

$$\tau_{\gamma,\alpha,i}^6 = \sum_{j \in O} Y_{j,\gamma}^2 \tau_{\alpha,i,j}^5 \quad (2r_T r_V N_o^2) \quad (9217)$$

$$\tau_{\gamma,i,a}^5 = \sum_{\alpha \in B} W_{a,\alpha}^1 \tau_{\gamma,\alpha}^4 \tau_{\gamma,\alpha,i}^3 \quad (3r_T r_V N_o N_v) \quad (9205)$$

$$\tau_{\gamma,\delta,\alpha,w}^7 = \sum_{i \in O} \tau_{\gamma,\alpha,i}^6 \tau_{\gamma,\delta,w,i}^3 \quad (2r_D r_T^2 r_V N_o) \quad (9218)$$

$$\tau_{\gamma,\delta,w}^6 = \sum_{i \in O} \sum_{a \in V} {}^2D_{a,w}^1 {}^2D_{i,w}^2 Y_{a,\delta}^{1,*} Y_{i,\delta}^{2,*} \tau_{\gamma,i,a}^5 \quad (5r_D r_T^2 N_o N_v) \quad (9206)$$

$$\tau_{\gamma,\alpha,w,i}^8 = \sum_{\delta \in A} \tau_{\delta,\alpha,i}^1 \tau_{\delta,\gamma,\alpha,w}^7 \quad (2r_D r_T^2 r_V N_o) \quad (9219)$$

$$\tau_{\gamma,\delta,w}^7 = \sum_{\epsilon \in A} Z_{\epsilon,\delta}^* \tau_{\gamma,\epsilon,w}^6 \quad (2r_D r_T^3) \quad (9207)$$

$$\tau_{\gamma,\alpha,w}^9 = \sum_{i \in O} {}^2D_{i,w}^4 Y_{i,\gamma}^{4,*} \tau_{\gamma,\alpha,w,i}^8 \quad (3r_D r_T r_V N_o) \quad (9220)$$

$$\tau_{\gamma,\delta,w}^8 = \sum_{\epsilon \in A} Z_{\epsilon,\gamma} \tau_{\epsilon,\delta,w}^7 \quad (2r_D r_T^3) \quad (9208)$$

$$\tau_{\gamma,w,a}^{10} = \sum_{\alpha \in B} W_{a,\alpha}^1 \tau_{\gamma,\alpha,w}^9 \quad (2r_D r_T r_V N_v) \quad (9221)$$

$${}^2R^3_{a,\gamma} \leftarrow - \sum_{w \in D} \frac{1}{2} {}^2D^3_{a,w} \tau^{10}_{\gamma,w,a} \quad (2r_D r_T N_v) \quad (9222)$$

Raw expression

$${}^2R^3_{b,\zeta} \leftarrow - \sum_{\gamma \in A} \sum_{i \in O} \sum_{j \in O} \sum_{k \in O} \sum_{a \in V} \sum_{c \in V} \sum_{d \in V} \frac{1}{2} {}^1T_{a,k} Y^{1,*}_{a,\gamma} Y^{2,*}_{i,\gamma} Z^*_{\gamma,\zeta} Y^{4,*}_{j,\zeta} {}^2D^{a,i,b,j} {}^2T_{c,j,d,i} V_{b,c,k,d} \quad (9223)$$

Factorized expression

$$\tau^0_{\gamma,\alpha} = \sum_{a \in V} W^2_{a,\alpha} Y^1_{a,\gamma} \quad (2r_T r_V N_v) \quad (9224)$$

$$\tau^1_{\gamma,\alpha,i} = \sum_{\delta \in A} Y^2_{i,\delta} Z_{\delta,\gamma} \tau^0_{\delta,\alpha} \quad (3r_T^2 r_V N_o) \quad (9225)$$

$$\tau^2_{\gamma,\delta,w} = \sum_{a \in V} {}^2D^1_{a,w} Y^3_{a,\gamma} Y^{1,*}_{a,\delta} \quad (3r_D r_T^2 N_v) \quad (9226)$$

$$\tau^3_{\gamma,\delta,w,i} = \sum_{\epsilon \in A} {}^2D^2_{i,w} Y^{2,*}_{i,\epsilon} Z^*_{\epsilon,\delta} \tau^2_{\gamma,\epsilon,w} \quad (4r_D r_T^3 N_o) \quad (9227)$$

$$\tau^4_{\alpha,i} = \sum_{a \in V} {}^1T_{a,i} W^4_{a,\alpha} \quad (2r_V N_o N_v) \quad (9228)$$

$$\tau^5_{\alpha,i,j} = \sum_{\beta \in B} X_{\alpha,\beta} W^3_{j,\beta} \tau^4_{\beta,i} \quad (3r_V^2 N_o^2) \quad (9229)$$

$$\tau^6_{\gamma,\alpha,i} = \sum_{j \in O} Y^4_{j,\gamma} \tau^5_{\alpha,i,j} \quad (2r_T r_V N_o^2) \quad (9230)$$

$$\tau^7_{\gamma,\delta,\alpha,w} = \sum_{i \in O} \tau^6_{\gamma,\alpha,i} \tau^3_{\gamma,\delta,w,i} \quad (2r_D r_T^2 r_V N_o) \quad (9231)$$

$$\tau^8_{\gamma,\alpha,w,i} = \sum_{\delta \in A} \tau^1_{\delta,\alpha,i} \tau^7_{\delta,\gamma,\alpha,w} \quad (2r_D r_T^2 r_V N_o) \quad (9232)$$

$$\tau^9_{\gamma,\alpha,w} = \sum_{i \in O} {}^2D^4_{i,w} Y^{4,*}_{i,\gamma} \tau^8_{\gamma,\alpha,w,i} \quad (3r_D r_T r_V N_o) \quad (9233)$$

$$\tau^{10}_{\gamma,w,a} = \sum_{\alpha \in B} W^1_{a,\alpha} \tau^9_{\gamma,\alpha,w} \quad (2r_D r_T r_V N_v) \quad (9234)$$

$${}^2R^3_{a,\gamma} \leftarrow - \sum_{w \in D} \frac{1}{2} {}^2D^3_{a,w} \tau^{10}_{\gamma,w,a} \quad (2r_D r_T N_v) \quad (9235)$$

Raw expression

$${}^2R^3_{b,\zeta} \leftarrow - \sum_{\gamma \in A} \sum_{i \in O} \sum_{j \in O} \sum_{k \in O} \sum_{a \in V} \sum_{c \in V} \sum_{d \in V} \frac{1}{2} {}^1T_{b,k} Y^{1,*}_{a,\gamma} Y^{2,*}_{i,\gamma} Z^*_{\gamma,\zeta} Y^{4,*}_{j,\zeta} {}^2D^{a,i,b,j} {}^2T_{c,i,d,j} V_{a,c,k,d} \quad (9236)$$

Factorized expression

$$\tau^0_{\gamma,\alpha,w} = \sum_{a \in V} {}^2D^1_{a,w} W^1_{a,\alpha} Y^{1,*}_{a,\gamma} \quad (3r_D r_T r_V N_v) \quad (9237)$$

$$\tau^1_{\gamma,\alpha} = \sum_{a \in V} W^2_{a,\alpha} Y^3_{a,\gamma} \quad (2r_T r_V N_v) \quad (9238)$$

$$\tau^2_{\gamma,\alpha,i} = \sum_{\delta \in A} Z_{\gamma,\delta} Y^4_{i,\delta} \tau^1_{\delta,\alpha} \quad (3r_T^2 r_V N_o) \quad (9239)$$

$$\tau^3_{\gamma,\delta,\alpha,w} = \sum_{i \in O} {}^2D^2_{i,w} Y^{2,*}_{i,\delta} \tau^0_{\delta,\alpha,w} \tau^2_{\gamma,\alpha,i} \quad (4r_D r_T^2 r_V N_o) \quad (9240)$$

$$\tau^4_{\alpha,i} = \sum_{a \in V} {}^1T_{a,i} W^4_{a,\alpha} \quad (2r_V N_o N_v) \quad (9241)$$

$$\tau^5_{\alpha,i,j} = \sum_{\beta \in B} X_{\alpha,\beta} W^3_{j,\beta} \tau^4_{\beta,i} \quad (3r_V^2 N_o^2) \quad (9242)$$

$$\tau^6_{\gamma,\alpha,i} = \sum_{j \in O} Y^2_{j,\gamma} \tau^5_{\alpha,i,j} \quad (2r_T r_V N_o^2) \quad (9243)$$

$$\tau^7_{\gamma,\delta,w,i} = \sum_{\alpha \in B} \tau^6_{\gamma,\alpha,i} \tau^3_{\gamma,\delta,\alpha,w} \quad (2r_D r_T^2 r_V N_o) \quad (9244)$$

$$\tau^8_{\gamma,\delta,w} = \sum_{\epsilon \in A} \sum_{i \in O} {}^2D^4_{i,w} Z^*_{\epsilon,\delta} Y^{4,*}_{i,\delta} \tau^7_{\gamma,\epsilon,w,i} \quad (4r_D r_T^3 N_o) \quad (9245)$$

$${}^2R^3_{a,\gamma} \leftarrow - \sum_{\delta \in A} \sum_{w \in D} \frac{1}{2} {}^2D^3_{a,w} Y^1_{a,\delta} \tau^8_{\delta,\gamma,w} \quad (3r_D r_T^2 N_v) \quad (9246)$$

Raw expression

$${}^2R^3_{b,\zeta} \leftarrow - \sum_{\gamma \in A} \sum_{i \in O} \sum_{j \in O} \sum_{k \in O} \sum_{a \in V} \sum_{c \in V} \sum_{d \in V} \frac{1}{2} {}^1T_{b,k} Y^{1,*}_{a,\gamma} Y^{2,*}_{i,\gamma} Z^*_{\gamma,\zeta} Y^{4,*}_{j,\zeta} {}^2D^{a,i,b,j} {}^2T_{c,j,d,i} V_{a,d,k,c} \quad (9247)$$

Factorized expression

$$\tau^0_{\gamma,\alpha,w} = \sum_{a \in V} {}^2D^1_{a,w} W^1_{a,\alpha} Y^{1,*}_{a,\gamma} \quad (3r_D r_T r_V N_v) \quad (9248)$$

$$\tau^1_{\gamma,\alpha} = \sum_{a \in V} W^2_{a,\alpha} Y^1_{a,\gamma} \quad (2r_T r_V N_v) \quad (9249)$$

$$\tau^2_{\gamma,\alpha,i} = \sum_{\delta \in A} Y^2_{i,\delta} Z_{\delta,\gamma} \tau^1_{\delta,\alpha} \quad (3r_T^2 r_V N_o) \quad (9250)$$

$$\tau^3_{\gamma,\delta,\alpha,w} = \sum_{i \in O} {}^2D^2_{i,w} Y^{2,*}_{i,\delta} \tau^0_{\delta,\alpha,w} \tau^2_{\gamma,\alpha,i} \quad (4r_D r_T^2 r_V N_o) \quad (9251)$$

$$\tau^4_{\alpha,i} = \sum_{a \in V} {}^1T_{a,i} W^4_{a,\alpha} \quad (2r_V N_o N_v) \quad (9252)$$

$$\tau^5_{\alpha,i,j} = \sum_{\beta \in B} X_{\alpha,\beta} W^3_{j,\beta} \tau^4_{\beta,i} \quad (3r_V^2 N_o^2) \quad (9253)$$

$$\tau^6_{\gamma,\alpha,i} = \sum_{j \in O} Y^4_{j,\gamma} \tau^5_{\alpha,i,j} \quad (2r_T r_V N_o^2) \quad (9254)$$

$$\tau^7_{\gamma,\delta,w,i} = \sum_{\alpha \in B} \tau^6_{\gamma,\alpha,i} \tau^3_{\gamma,\delta,\alpha,w} \quad (2r_D r_T^2 r_V N_o) \quad (9255)$$

$$\tau^8_{\gamma,\delta,w} = \sum_{\epsilon \in A} \sum_{i \in O} {}^2D^4_{i,w} Z^*_{\epsilon,\delta} Y^{4,*}_{i,\delta} \tau^7_{\gamma,\epsilon,w,i} \quad (4r_D r_T^3 N_o) \quad (9256)$$

$${}^2R^3_{a,\gamma} \leftarrow - \sum_{\delta \in A} \sum_{w \in D} \frac{1}{2} {}^2D^3_{a,w} Y^3_{a,\delta} \tau^8_{\delta,\gamma,w} \quad (3r_D r_T^2 N_v) \quad (9257)$$

Raw expression

$${}^2R^3_{b,\zeta} \leftarrow - \sum_{\gamma \in A} \sum_{i \in O} \sum_{j \in O} \sum_{k \in O} \sum_{a \in V} \sum_{c \in V} \sum_{d \in V} \frac{1}{2} {}^1T_{c,i} Y^{1,*}_{a,\gamma} Y^{2,*}_{i,\gamma} Z^*_{\gamma,\zeta} Y^{4,*}_{j,\zeta} {}^2D^{a,i,b,j} {}^2T_{a,k,d,j} V_{b,d,k,c} \quad (9258)$$

Factorized expression

$$\tau^0_{\alpha,i} = \sum_{a \in V} {}^1T_{a,i} W^2_{a,\alpha} \quad (2r_V N_o N_v) \quad (9259)$$

$$\tau^1_{\gamma,\alpha,w} = \sum_{i \in O} {}^2D^4_{i,w} Y^{4,*}_{i,\gamma} \tau^0_{\alpha,i} \quad (3r_D r_T r_V N_o) \quad (9260)$$

$$\tau^2_{\gamma,\delta,w} = \sum_{a \in V} {}^2D^1_{a,w} Y^1_{a,\gamma} Y^{1,*}_{a,\delta} \quad (3r_D r_T^2 N_v) \quad (9261)$$

$$\tau^3_{\gamma,\alpha} = \sum_{i \in O} W^3_{i,\alpha} Y^2_{i,\gamma} \quad (2r_T r_V N_o) \quad (9262)$$

$$\tau^4_{\gamma,\alpha} = \sum_{a \in V} W^4_{a,\alpha} Y^3_{a,\gamma} \quad (2r_T r_V N_v) \quad (9263)$$

$$\tau^5_{\gamma,\alpha,i} = \sum_{\delta \in A} Z_{\gamma,\delta} Y^4_{i,\delta} \tau^4_{\delta,\alpha} \quad (3r_T^2 r_V N_o) \quad (9264)$$

$$\tau^6_{\gamma,\alpha,w} = \sum_{\delta \in A} \sum_{i \in O} {}^2D^2_{i,w} Y^{2,*}_{i,\gamma} \tau^3_{\delta,\alpha} \tau^2_{\delta,\gamma,w} \tau^5_{\delta,\alpha,i} \quad (5r_D r_T^2 r_V N_o) \quad (9265)$$

$$\tau^7_{\gamma,\alpha,w} = \sum_{\beta \in B} X_{\alpha,\beta} \tau^6_{\gamma,\beta,w} \quad (2r_D r_T r_V^2) \quad (9266)$$

$$\tau^8_{\gamma,\alpha,w} = \sum_{\delta \in A} Z^*_{\delta,\gamma} \tau^7_{\delta,\alpha,w} \quad (2r_D r_T^2 r_V) \quad (9267)$$

$$\tau^9_{\gamma,w,a} = \sum_{\alpha \in B} W^1_{a,\alpha} \tau^1_{\gamma,\alpha,w} \tau^8_{\gamma,\alpha,w} \quad (3r_D r_T r_V N_v) \quad (9268)$$

$${}^2R^3_{a,\gamma} \leftarrow - \sum_{w \in D} \frac{1}{2} {}^2D^3_{a,w} \tau^9_{\gamma,w,a} \quad (2r_D r_T N_v) \quad (9269)$$

Raw expression

$${}^2R^3_{b,\zeta} \leftarrow - \sum_{\gamma \in A} \sum_{i \in O} \sum_{j \in O} \sum_{k \in O} \sum_{a \in V} \sum_{c \in V} \sum_{d \in V} \frac{1}{2} {}^1T_{c,i} Y^{1,*}_{a,\gamma} Y^{2,*}_{i,\gamma} Z^*_{\gamma,\zeta} Y^{4,*}_{j,\zeta} {}^2D^{a,i,b,j} {}^2T_{b,j,d,k} V_{a,d,k,c} \quad (9270)$$

Factorized expression

$$\tau^0_{\alpha,i} = \sum_{a \in V} {}^1T_{a,i} W^2_{a,\alpha} \quad (2r_V N_o N_v) \quad (9271)$$

$$\tau^1_{\gamma,\alpha,w} = \sum_{i \in O} {}^2D^4_{i,w} Y^{4,*}_{i,\gamma} \tau^0_{\alpha,i} \quad (3r_D r_T r_V N_o) \quad (9272)$$

$$\tau^2_{\gamma,\delta,w} = \sum_{\epsilon \in A} Z^*_{\epsilon,\delta} \tau^0_{\gamma,\epsilon,w} \tau^1_{\gamma,\epsilon,w} \quad (3r_D r_T^3) \quad (9285)$$

$$\tau^2_{\gamma,\delta,w} = \sum_{a \in V} {}^2D^1_{a,w} Y^3_{a,\gamma} Y^{1,*}_{a,\delta} \quad (3r_D r_T^2 N_v) \quad (9273)$$

$$\tau^3_{\gamma,\delta,w} = \sum_{\epsilon \in A} Z_{\epsilon,\gamma} \tau^2_{\epsilon,\delta,w} \quad (2r_D r_T^3) \quad (9286)$$

$$\tau^3_{\gamma,\alpha} = \sum_{a \in V} W^4_{a,\alpha} Y^1_{a,\gamma} \quad (2r_T r_V N_v) \quad (9274)$$

$$\tau^4_{\alpha,i} = \sum_{a \in V} {}^1T_{a,i} W^4_{a,\alpha} \quad (2r_V N_o N_v) \quad (9287)$$

$$\tau^4_{\gamma,\alpha,i} = \sum_{\delta \in A} Y^2_{i,\delta} Z_{\delta,\gamma} \tau^3_{\delta,\alpha} \quad (3r_T^2 r_V N_o) \quad (9275)$$

$$\tau^5_{\alpha,i,j} = \sum_{\beta \in B} X_{\alpha,\beta} W^3_{j,\beta} \tau^4_{\beta,i} \quad (3r_V^2 N_o^2) \quad (9288)$$

$$\tau^5_{\gamma,\alpha} = \sum_{i \in O} W^3_{i,\alpha} Y^4_{i,\gamma} \quad (2r_T r_V N_o) \quad (9276)$$

$$\tau^6_{\gamma,\alpha,i} = \sum_{j \in O} Y^4_{j,\gamma} \tau^5_{\alpha,i,j} \quad (2r_T r_V N_o^2) \quad (9289)$$

$$\tau^6_{\gamma,\alpha,w} = \sum_{\delta \in A} \sum_{i \in O} {}^2D^2_{i,w} Y^{2,*}_{i,\gamma} \tau^5_{\delta,\alpha} \tau^2_{\delta,\gamma,w} \tau^4_{\delta,\alpha,i} \quad (5r_D r_T^2 r_V N_o) \quad (9277)$$

$$\tau^7_{\gamma,\alpha} = \sum_{a \in V} W^2_{a,\alpha} Y^3_{a,\gamma} \quad (2r_T r_V N_v) \quad (9290)$$

$$\tau^7_{\gamma,\alpha,w} = \sum_{\beta \in B} X_{\alpha,\beta} \tau^6_{\gamma,\beta,w} \quad (2r_D r_T r_V^2) \quad (9278)$$

$$\tau^8_{\gamma,i,a} = \sum_{\alpha \in B} W^1_{a,\alpha} \tau^7_{\gamma,\alpha} \tau^6_{\gamma,\alpha,i} \quad (3r_T r_V N_o N_v) \quad (9291)$$

$$\tau^8_{\gamma,\alpha,w} = \sum_{\delta \in A} Z^*_{\delta,\gamma} \tau^7_{\delta,\alpha,w} \quad (2r_D r_T^2 r_V) \quad (9279)$$

$$\tau^9_{\gamma,w,a} = \sum_{\delta \in A} \sum_{i \in O} {}^2D^4_{i,w} Y^{4,*}_{i,\gamma} \tau^3_{\delta,\gamma,w} \tau^8_{\delta,i,a} \quad (4r_D r_T^2 N_o N_v) \quad (9292)$$

$$\tau^9_{\gamma,w,a} = \sum_{\alpha \in B} W^1_{a,\alpha} \tau^1_{\gamma,\alpha,w} \tau^8_{\gamma,\alpha,w} \quad (3r_D r_T r_V N_v) \quad (9280)$$

$${}^2R^3_{a,\gamma} \leftarrow - \sum_{w \in D} \frac{1}{2} {}^2D^3_{a,w} \tau^9_{\gamma,w,a} \quad (2r_D r_T N_v) \quad (9293)$$

Raw expression

$${}^2R^3_{a,\gamma} \leftarrow - \sum_{w \in D} \frac{1}{2} {}^2D^3_{a,w} \tau^9_{\gamma,w,a} \quad (2r_D r_T N_v) \quad (9281)$$

$${}^2R^3_{b,\zeta} \leftarrow - \sum_{\gamma \in A} \sum_{i \in O} \sum_{j \in O} \sum_{k \in O} \sum_{a \in V} \sum_{c \in V} \sum_{d \in V} \frac{1}{2} {}^1T_{c,i} Y^{1,*}_{a,\gamma} Y^{2,*}_{i,\gamma} Z^*_{\gamma,\zeta} Y^{4,*}_{j,\zeta} {}^2D^{a,i,b,j} {}^2T_{d,j,a,k} V_{b,d,k,c} \quad (9294)$$

Raw expression

$${}^2R^3_{b,\zeta} \leftarrow - \sum_{\gamma \in A} \sum_{i \in O} \sum_{j \in O} \sum_{k \in O} \sum_{a \in V} \sum_{c \in V} \sum_{d \in V} \frac{1}{2} {}^1T_{c,i} Y^{1,*}_{a,\gamma} Y^{2,*}_{i,\gamma} Z^*_{\gamma,\zeta} Y^{4,*}_{j,\zeta} {}^2D^{a,i,b,j} {}^2T_{b,k,d,j} V_{a,c,k,d} \quad (9282)$$

Factorized expression

Factorized expression

$$\tau^0_{\gamma,\delta,w} = \sum_{a \in V} {}^2D^1_{a,w} Y^1_{a,\gamma} Y^{1,*}_{a,\delta} \quad (3r_D r_T^2 N_v) \quad (9283)$$

$$\tau^1_{\gamma,\delta,w} = \sum_{i \in O} {}^2D^2_{i,w} Y^4_{i,\gamma} Y^{2,*}_{i,\delta} \quad (3r_D r_T^2 N_o) \quad (9296)$$

$$\tau^1_{\gamma,\delta,w} = \sum_{i \in O} {}^2D^2_{i,w} Y^2_{i,\gamma} Y^{2,*}_{i,\delta} \quad (3r_D r_T^2 N_o) \quad (9284)$$

$$\tau^2_{\gamma,\delta,w} = \sum_{\epsilon \in A} Z^*_{\epsilon,\delta} \tau^0_{\gamma,\epsilon,w} \tau^1_{\gamma,\epsilon,w} \quad (3r_D r_T^3) \quad (9297)$$

$$\tau_{\gamma,\delta,w}^3 = \sum_{\epsilon \in A} Z_{\gamma,\epsilon} \tau_{\epsilon,\delta,w}^2 \quad (2r_D r_T^3) \quad (9298)$$

$$\tau_{\alpha,a}^4 = \sum_{\beta \in B} X_{\alpha,\beta} W_{a,\beta}^4 \tau_{\alpha,\beta}^3 \quad (3r_V^2 N_v) \quad (9311)$$

$$\tau_{\alpha,i}^4 = \sum_{a \in V} {}^1T_{a,i} W_{a,\alpha}^4 \quad (2r_V N_o N_v) \quad (9299)$$

$$\tau_{a,b}^5 = \sum_{\alpha \in B} W_{a,\alpha}^1 \tau_{\alpha,b}^4 \quad (2r_V N_v^2) \quad (9312)$$

$$\tau_{\alpha,i,j}^5 = \sum_{\beta \in B} X_{\alpha,\beta} W_{j,\beta}^3 \tau_{\beta,i}^4 \quad (3r_V^2 N_o^2) \quad (9300)$$

$$\tau_{\gamma,a}^6 = \sum_{b \in V} Y_{b,\gamma}^3 \tau_{a,b}^5 \quad (2r_T N_v^2) \quad (9313)$$

$$\tau_{\gamma,\alpha,i}^6 = \sum_{j \in O} Y_{j,\gamma}^2 \tau_{\alpha,i,j}^5 \quad (2r_T r_V N_o^2) \quad (9301)$$

$$\tau_{\gamma,\delta,w}^7 = \sum_{a \in V} {}^2D_{a,w}^1 Y_{a,\delta}^{1,*} \tau_{\gamma,a}^6 \quad (3r_D r_T^2 N_v) \quad (9314)$$

$$\tau_{\gamma,\alpha}^7 = \sum_{a \in V} W_{a,\alpha}^2 Y_{a,\gamma}^1 \quad (2r_T r_V N_v) \quad (9302)$$

$$\tau_{\gamma,\delta,w}^8 = \sum_{\epsilon \in A} Z_{\epsilon,\delta}^* \tau_{\gamma,\epsilon,w}^1 \tau_{\gamma,\epsilon,w}^7 \quad (3r_D r_T^3) \quad (9315)$$

$$\tau_{\gamma,i,a}^8 = \sum_{\alpha \in B} W_{a,\alpha}^1 \tau_{\gamma,\alpha}^7 \tau_{\gamma,\alpha,i}^6 \quad (3r_T r_V N_o N_v) \quad (9303)$$

$$\tau_{\gamma,\delta,w}^9 = \sum_{\epsilon \in A} Z_{\gamma,\epsilon} \tau_{\epsilon,\delta,w}^8 \quad (2r_D r_T^3) \quad (9316)$$

$$\tau_{\gamma,w,a}^9 = \sum_{\delta \in A} \sum_{i \in O} {}^2D_{i,w}^4 Y_{i,\gamma}^{4,*} \tau_{\delta,\gamma,w}^3 \tau_{\delta,i,a}^8 \quad (4r_D r_T^2 N_o N_v)^2 R_{a,\gamma}^3 \leftarrow - \sum_{\delta \in A} \sum_{w \in D} \frac{1}{2} {}^2D_{a,w}^3 Y_{a,\delta}^1 \tau_{\delta,\gamma,w}^0 \tau_{\delta,\gamma,w}^9 \quad (4r_D r_T^2 N_v) \quad (9304) \quad (9317)$$

$${}^2R_{a,\gamma}^3 \leftarrow - \sum_{w \in D} \frac{1}{2} {}^2D_{a,w}^3 \tau_{\gamma,w,a}^9 \quad (2r_D r_T N_v) \quad (9305)$$

Raw expression

$${}^2R_{b,\zeta}^3 \leftarrow - \sum_{\gamma \in A} \sum_{i \in O} \sum_{j \in O} \sum_{k \in O} \sum_{a \in V} \sum_{c \in V} \sum_{d \in V} \frac{1}{2} {}^1T_{c,i} Y_{a,\gamma}^{1,*} Y_{i,\gamma}^{2,*} Z_{\gamma,\zeta}^* Y_{j,\zeta}^{4,*} {}^2D_{a,i,b,j} {}^2T_{d,k,b,j} V_{a,d,k,c} \quad (9318)$$

Raw expression

$${}^2R_{b,\zeta}^3 \leftarrow - \sum_{\gamma \in A} \sum_{i \in O} \sum_{j \in O} \sum_{k \in O} \sum_{a \in V} \sum_{c \in V} \sum_{d \in V} \frac{1}{2} {}^1T_{c,i} Y_{a,\gamma}^{1,*} Y_{i,\gamma}^{2,*} Z_{\gamma,\zeta}^* Y_{j,\zeta}^{4,*} {}^2D_{a,i,b,j} {}^2T_{d,j,b,k} V_{a,c,k,d} \quad (9306)$$

Factorized expression

$$\tau_{\gamma,\delta,w}^0 = \sum_{i \in O} {}^2D_{i,w}^4 Y_{i,\gamma}^4 Y_{i,\delta}^{4,*} \quad (3r_D r_T^2 N_o) \quad (9319)$$

Factorized expression

$$\tau_{\gamma,\delta,w}^0 = \sum_{i \in O} {}^2D_{i,w}^4 Y_{i,\gamma}^2 Y_{i,\delta}^{4,*} \quad (3r_D r_T^2 N_o) \quad (9307)$$

$$\tau_{\gamma,\delta,w}^1 = \sum_{i \in O} {}^2D_{i,w}^2 Y_{i,\gamma}^2 Y_{i,\delta}^{2,*} \quad (3r_D r_T^2 N_o) \quad (9320)$$

$$\tau_{\gamma,\delta,w}^1 = \sum_{i \in O} {}^2D_{i,w}^2 Y_{i,\gamma}^4 Y_{i,\delta}^{2,*} \quad (3r_D r_T^2 N_o) \quad (9308)$$

$$\tau_{\alpha,i}^2 = \sum_{a \in V} {}^1T_{a,i} W_{a,\alpha}^2 \quad (2r_V N_o N_v) \quad (9321)$$

$$\tau_{\alpha,i}^2 = \sum_{a \in V} {}^1T_{a,i} W_{a,\alpha}^2 \quad (2r_V N_o N_v) \quad (9309)$$

$$\tau_{\alpha,\beta}^3 = \sum_{i \in O} W_{i,\beta}^3 \tau_{\alpha,i}^2 \quad (2r_V^2 N_o) \quad (9322)$$

$$\tau_{\alpha,\beta}^3 = \sum_{i \in O} W_{i,\beta}^3 \tau_{\alpha,i}^2 \quad (2r_V^2 N_o) \quad (9310)$$

$$\tau_{\alpha,a}^4 = \sum_{\beta \in B} X_{\alpha,\beta} W_{a,\beta}^4 \tau_{\alpha,\beta}^3 \quad (3r_V^2 N_v) \quad (9323)$$

$$\tau^5_{a,b} = \sum_{\alpha \in B} W^1_{a,\alpha} \tau^4_{\alpha,b} \quad (2r_V N_v^2) \quad (9324)$$

$$\tau^6_{\gamma,\delta,w} = \sum_{a \in V} {}^2D^1_{a,w} Y^1_{a,\gamma} Y^{1,*}_{a,\delta} \quad (3r_D r_T^2 N_v) \quad (9337)$$

$$\tau^6_{\gamma,a} = \sum_{b \in V} Y^1_{b,\gamma} \tau^5_{a,b} \quad (2r_T N_v^2) \quad (9325)$$

$$\tau^7_{\gamma,\delta,w} = \sum_{i \in O} {}^2D^2_{i,w} Y^2_{i,\gamma} Y^{2,*}_{i,\delta} \quad (3r_D r_T^2 N_o) \quad (9338)$$

$$\tau^7_{\gamma,\delta,w} = \sum_{a \in V} {}^2D^1_{a,w} Y^{1,*}_{a,\delta} \tau^6_{\gamma,a} \quad (3r_D r_T^2 N_v) \quad (9326)$$

$$\tau^8_{\gamma,\delta,w} = \sum_{\epsilon \in A} Z^*_{\epsilon,\delta} \tau^6_{\gamma,\epsilon,w} \tau^7_{\gamma,\epsilon,w} \quad (3r_D r_T^3) \quad (9339)$$

$$\tau^8_{\gamma,\delta,w} = \sum_{\epsilon \in A} Z^*_{\epsilon,\delta} \tau^1_{\gamma,\epsilon,w} \tau^7_{\gamma,\epsilon,w} \quad (3r_D r_T^3) \quad (9327)$$

$$\tau^9_{\gamma,\delta,w} = \sum_{\epsilon \in A} Z_{\epsilon,\gamma} \tau^8_{\epsilon,\delta,w} \quad (2r_D r_T^3) \quad (9340)$$

$$\tau^9_{\gamma,\delta,w} = \sum_{\epsilon \in A} Z_{\epsilon,\gamma} \tau^8_{\epsilon,\delta,w} \quad (2r_D r_T^3) \quad (9328)$$

$${}^2R^3_{a,\gamma} \leftarrow - \sum_{\delta \in A} \sum_{w \in D} \frac{1}{2} {}^2D^3_{a,w} \tau^4_{\delta,a} \tau^5_{\delta,\gamma,w} \tau^9_{\delta,\gamma,w} \quad (4r_D r_T^2 N_v) \quad (9341)$$

$${}^2R^3_{a,\gamma} \leftarrow - \sum_{\delta \in A} \sum_{w \in D} \frac{1}{2} {}^2D^3_{a,w} Y^3_{a,\delta} \tau^0_{\delta,\gamma,w} \tau^9_{\delta,\gamma,w} \quad (4r_D r_T^2 N_v) \text{Raw expression} \quad (9329)$$

Raw expression

$${}^2R^3_{b,\zeta} \leftarrow - \sum_{\gamma \in A} \sum_{i \in O} \sum_{j \in O} \sum_{k \in O} \sum_{a \in V} \sum_{c \in V} \sum_{d \in V} \frac{1}{2} {}^1T_{c,j} Y^{1,*}_{a,\gamma} Y^{2,*}_{i,\gamma} Z^*_{\gamma,\zeta} Y^{4,*}_{j,\zeta} {}^2D^{a,i,b,j} {}^2T_{a,i,d,k} V_{b,d,k,c} \quad (9330)$$

Factorized expression

$${}^2R^3_{b,\zeta} \leftarrow - \sum_{\gamma \in A} \sum_{i \in O} \sum_{j \in O} \sum_{k \in O} \sum_{a \in V} \sum_{c \in V} \sum_{d \in V} \frac{1}{2} {}^1T_{c,j} Y^{1,*}_{a,\gamma} Y^{2,*}_{i,\gamma} Z^*_{\gamma,\zeta} Y^{4,*}_{j,\zeta} {}^2D^{a,i,b,j} {}^2T_{a,k,d,i} V_{b,c,k,d} \quad (9342)$$

Factorized expression

$$\tau^0_{\alpha,i} = \sum_{a \in V} {}^1T_{a,i} W^2_{a,\alpha} \quad (2r_V N_o N_v) \quad (9343)$$

$$\tau^0_{\alpha,i} = \sum_{a \in V} {}^1T_{a,i} W^2_{a,\alpha} \quad (2r_V N_o N_v) \quad (9331)$$

$$\tau^1_{\alpha,\beta} = \sum_{i \in O} W^3_{i,\beta} \tau^0_{\alpha,i} \quad (2r_V^2 N_o) \quad (9344)$$

$$\tau^1_{\alpha,\beta} = \sum_{i \in O} W^3_{i,\beta} \tau^0_{\alpha,i} \quad (2r_V^2 N_o) \quad (9332)$$

$$\tau^2_{\alpha,a} = \sum_{\beta \in B} X_{\alpha,\beta} W^4_{a,\beta} \tau^1_{\alpha,\beta} \quad (3r_V^2 N_v) \quad (9345)$$

$$\tau^2_{\alpha,a} = \sum_{\beta \in B} X_{\alpha,\beta} W^4_{a,\beta} \tau^1_{\alpha,\beta} \quad (3r_V^2 N_v) \quad (9333)$$

$$\tau^3_{a,b} = \sum_{\alpha \in B} W^1_{a,\alpha} \tau^2_{\alpha,b} \quad (2r_V N_v^2) \quad (9346)$$

$$\tau^3_{a,b} = \sum_{\alpha \in B} W^1_{a,\alpha} \tau^2_{\alpha,b} \quad (2r_V N_v^2) \quad (9334)$$

$$\tau^4_{\gamma,a} = \sum_{b \in V} Y^1_{b,\gamma} \tau^3_{a,b} \quad (2r_T N_v^2) \quad (9347)$$

$$\tau^4_{\gamma,a} = \sum_{b \in V} Y^3_{b,\gamma} \tau^3_{a,b} \quad (2r_T N_v^2) \quad (9335)$$

$$\tau^5_{\gamma,\delta,w} = \sum_{i \in O} {}^2D^4_{i,w} Y^2_{i,\gamma} Y^{4,*}_{i,\delta} \quad (3r_D r_T^2 N_o) \quad (9348)$$

$$\tau^5_{\gamma,\delta,w} = \sum_{i \in O} {}^2D^4_{i,w} Y^4_{i,\gamma} Y^{4,*}_{i,\delta} \quad (3r_D r_T^2 N_o) \quad (9336)$$

$$\tau^6_{\gamma,\delta,w} = \sum_{a \in V} {}^2D^1_{a,w} Y^3_{a,\gamma} Y^{1,*}_{a,\delta} \quad (3r_D r_T^2 N_v) \quad (9349)$$

Raw expression

$$\tau^7_{\gamma,\delta,w} = \sum_{i \in O} {}^2D^2_{i,w} Y^4_{i,\gamma} Y^{2,*}_{i,\delta} \quad (3r_D r_T^2 N_o) \quad (9350)$$

$$\tau^8_{\gamma,\delta,w} = \sum_{\epsilon \in A} Z^*_{\epsilon,\delta} \tau^6_{\gamma,\epsilon,w} \tau^7_{\gamma,\epsilon,w} \quad (3r_D r_T^3) \quad (9351)$$

$$\tau^9_{\gamma,\delta,w} = \sum_{\epsilon \in A} Z_{\gamma,\epsilon} \tau^8_{\epsilon,\delta,w} \quad (2r_D r_T^3) \quad (9352)$$

$${}^2R^3_{a,\gamma} \leftarrow - \sum_{\delta \in A} \sum_{w \in D} \frac{1}{2} {}^2D^3_{a,w} \tau^4_{\delta,a} \tau^5_{\delta,\gamma,w} \tau^9_{\delta,\gamma,w} \quad (4r_D r_T^2 N_v) \quad (9353)$$

Raw expression

$${}^2R^3_{b,\zeta} \leftarrow - \sum_{\gamma \in A} \sum_{i \in O} \sum_{j \in O} \sum_{k \in O} \sum_{a \in V} \sum_{c \in V} \sum_{d \in V} \frac{1}{2} {}^1T_{c,j} Y^{1,*}_{a,\gamma} Y^{2,*}_{i,\gamma} Z^*_{\gamma,\zeta} Y^{4,*}_{j,\zeta} {}^2D^{a,i,b,j} {}^2T_{b,k,d,i} V_{a,d,k,c} \quad (9354)$$

Factorized expression

$$\tau^0_{\gamma,\delta,w} = \sum_{i \in O} {}^2D^4_{i,w} Y^2_{i,\gamma} Y^{4,*}_{i,\delta} \quad (3r_D r_T^2 N_o) \quad (9355)$$

$$\tau^1_{\gamma,\delta,w} = \sum_{i \in O} {}^2D^2_{i,w} Y^4_{i,\gamma} Y^{2,*}_{i,\delta} \quad (3r_D r_T^2 N_o) \quad (9356)$$

$$\tau^2_{\gamma,w,i} = \sum_{a \in V} {}^2D^1_{a,w} {}^1T_{a,i} Y^{1,*}_{a,\gamma} \quad (3r_D r_T N_o N_v) \quad (9357)$$

$$\tau^3_{\gamma,i} = \sum_{a \in V} Y^3_{a,\gamma} f_{i,a} \quad (2r_T N_o N_v) \quad (9358)$$

$$\tau^4_{\gamma,\delta,w} = \sum_{i \in O} \tau^3_{\gamma,i} \tau^2_{\delta,w,i} \quad (2r_D r_T^2 N_o) \quad (9359)$$

$$\tau^5_{\gamma,\delta,w} = \sum_{\epsilon \in A} Z^*_{\epsilon,\delta} \tau^1_{\gamma,\epsilon,w} \tau^4_{\gamma,\epsilon,w} \quad (3r_D r_T^3) \quad (9360)$$

$$\tau^6_{\gamma,\delta,w} = \sum_{\epsilon \in A} Z_{\gamma,\epsilon} \tau^5_{\epsilon,\delta,w} \quad (2r_D r_T^3) \quad (9361)$$

$${}^2R^3_{a,\gamma} \leftarrow - \sum_{\delta \in A} \sum_{w \in D} \frac{1}{2} {}^2D^3_{a,w} Y^1_{a,\delta} \tau^0_{\delta,\gamma,w} \tau^6_{\delta,\gamma,w} \quad (4r_D r_T^2 N_v) \quad (9362)$$

$${}^2R^3_{b,\zeta} \leftarrow - \sum_{\gamma \in A} \sum_{i \in O} \sum_{j \in O} \sum_{k \in O} \sum_{a \in V} \sum_{c \in V} \sum_{d \in V} \frac{1}{2} {}^1T_{c,j} Y^{1,*}_{a,\gamma} Y^{2,*}_{i,\gamma} Z^*_{\gamma,\zeta} Y^{4,*}_{j,\zeta} {}^2D^{a,i,b,j} {}^2T_{d,i,a,k} V_{b,c,k,d} \quad (9363)$$

Factorized expression

$$\tau^0_{\gamma,\delta,w} = \sum_{i \in O} {}^2D^2_{i,w} Y^2_{i,\gamma} Y^{2,*}_{i,\delta} \quad (3r_D r_T^2 N_o) \quad (9364)$$

$$\tau^1_{\gamma,w,i} = \sum_{a \in V} {}^2D^1_{a,w} {}^1T_{a,i} Y^{1,*}_{a,\gamma} \quad (3r_D r_T N_o N_v) \quad (9365)$$

$$\tau^2_{\gamma,i} = \sum_{a \in V} Y^1_{a,\gamma} f_{i,a} \quad (2r_T N_o N_v) \quad (9366)$$

$$\tau^3_{\gamma,\delta,w} = \sum_{i \in O} \tau^2_{\gamma,i} \tau^1_{\delta,w,i} \quad (2r_D r_T^2 N_o) \quad (9367)$$

$$\tau^4_{\gamma,\delta,w} = \sum_{\epsilon \in A} Z^*_{\epsilon,\delta} \tau^0_{\gamma,\epsilon,w} \tau^3_{\gamma,\epsilon,w} \quad (3r_D r_T^3) \quad (9368)$$

$$\tau^5_{\gamma,\delta,w} = \sum_{\epsilon \in A} Z_{\epsilon,\gamma} \tau^4_{\epsilon,\delta,w} \quad (2r_D r_T^3) \quad (9369)$$

$$\tau^6_{\gamma,\delta,w} = \sum_{i \in O} {}^2D^4_{i,w} Y^4_{i,\gamma} Y^{4,*}_{i,\delta} \quad (3r_D r_T^2 N_o) \quad (9370)$$

$${}^2R^3_{a,\gamma} \leftarrow - \sum_{\delta \in A} \sum_{w \in D} \frac{1}{2} {}^2D^3_{a,w} Y^3_{a,\delta} \tau^5_{\delta,\gamma,w} \tau^6_{\delta,\gamma,w} \quad (4r_D r_T^2 N_v) \quad (9371)$$

Raw expression

$${}^2R^3_{b,\zeta} \leftarrow - \sum_{\gamma \in A} \sum_{i \in O} \sum_{j \in O} \sum_{k \in O} \sum_{a \in V} \sum_{c \in V} \sum_{d \in V} \frac{1}{2} {}^1T_{c,j} Y^{1,*}_{a,\gamma} Y^{2,*}_{i,\gamma} Z^*_{\gamma,\zeta} Y^{4,*}_{j,\zeta} {}^2D^{a,i,b,j} {}^2T_{d,i,b,k} V_{a,d,k,c} \quad (9372)$$

Factorized expression

$$\tau^0_{\gamma,\delta,w} = \sum_{i \in O} {}^2D^4_{i,w} Y^4_{i,\gamma} Y^{4,*}_{i,\delta} \quad (3r_D r_T^2 N_o) \quad (9373)$$

$$\tau^1_{\gamma,\delta,w} = \sum_{a \in V} {}^2D^1_{a,w} Y^1_{a,\gamma} Y^{1,*}_{a,\delta} \quad (3r_D r_T^2 N_v) \quad (9374)$$



$$\tau_{\gamma,\delta,w}^2 = \sum_{i \in O} {}^2D_{i,w}^2 Y_{i,\gamma}^2 Y_{i,\delta}^{2,*} \quad (3r_D r_T^2 N_o) \quad (9375)$$

$$\tau_{\gamma,\delta,w}^3 = \sum_{\epsilon \in A} Z_{\epsilon,\delta}^* \tau_{\gamma,\epsilon,w}^1 \tau_{\gamma,\epsilon,w}^2 \quad (3r_D r_T^3) \quad (9376)$$

$$\tau_{\gamma,\delta,w}^4 = \sum_{\epsilon \in A} Z_{\epsilon,\gamma} \tau_{\epsilon,\delta,w}^3 \quad (2r_D r_T^3) \quad (9377)$$

$$\tau_{\gamma,i}^5 = \sum_{a \in V} Y_{a,\gamma}^3 f_{i,a} \quad (2r_T N_o N_v) \quad (9378)$$

$$\tau_{\gamma,w,i}^6 = \sum_{\delta \in A} \tau_{\delta,i}^5 \tau_{\delta,\gamma,w}^0 \tau_{\delta,\gamma,w}^4 \quad (3r_D r_T^2 N_o) \quad (9379)$$

$${}^2R_{a,\gamma}^3 \leftarrow - \sum_{w \in D} \sum_{i \in O} \frac{1}{2} {}^2D_{a,w}^3 T_{a,i} \tau_{\gamma,w,i}^6 \quad (3r_D r_T N_o N_v) \quad (9380)$$

Raw expression

$${}^2R_{b,\zeta}^3 \leftarrow - \sum_{\gamma \in A} \sum_{i \in O} \sum_{j \in O} \sum_{k \in O} \sum_{a \in V} \sum_{c \in V} \sum_{d \in V} \frac{1}{2} {}^1T_{c,j} Y_{a,\gamma}^{1,*} Y_{i,\gamma}^{2,*} Z_{\gamma,\zeta}^* Y_{j,\zeta}^{4,*} {}^2D_{a,i,b,j} {}^2T_{d,k,a,i} V_{b,d,k,c} \quad (9381)$$

Factorized expression

$$\tau_{\gamma,\delta,w}^0 = \sum_{i \in O} {}^2D_{i,w}^4 Y_{i,\gamma}^2 Y_{i,\delta}^{4,*} \quad (3r_D r_T^2 N_o) \quad (9382)$$

$$\tau_{\gamma,\delta,w}^1 = \sum_{a \in V} {}^2D_{a,w}^1 Y_{a,\gamma}^3 Y_{a,\delta}^{1,*} \quad (3r_D r_T^2 N_v) \quad (9383)$$

$$\tau_{\gamma,\delta,w}^2 = \sum_{i \in O} {}^2D_{i,w}^2 Y_{i,\gamma}^4 Y_{i,\delta}^{2,*} \quad (3r_D r_T^2 N_o) \quad (9384)$$

$$\tau_{\gamma,\delta,w}^3 = \sum_{\epsilon \in A} Z_{\epsilon,\delta}^* \tau_{\gamma,\epsilon,w}^1 \tau_{\gamma,\epsilon,w}^2 \quad (3r_D r_T^3) \quad (9385)$$

$$\tau_{\gamma,\delta,w}^4 = \sum_{\epsilon \in A} Z_{\gamma,\epsilon} \tau_{\epsilon,\delta,w}^3 \quad (2r_D r_T^3) \quad (9386)$$

$$\tau_{\gamma,i}^5 = \sum_{a \in V} Y_{a,\gamma}^1 f_{i,a} \quad (2r_T N_o N_v) \quad (9387)$$

$$\tau_{\gamma,w,i}^6 = \sum_{\delta \in A} \tau_{\delta,i}^5 \tau_{\delta,\gamma,w}^0 \tau_{\delta,\gamma,w}^4 \quad (3r_D r_T^2 N_o) \quad (9388)$$

$${}^2R_{a,\gamma}^3 \leftarrow - \sum_{w \in D} \sum_{i \in O} \frac{1}{2} {}^2D_{a,w}^3 T_{a,i} \tau_{\gamma,w,i}^6 \quad (3r_D r_T N_o N_v) \quad (9389)$$

Raw expression

$${}^2R_{b,\zeta}^3 \leftarrow - \sum_{\gamma \in A} \sum_{i \in O} \sum_{j \in O} \sum_{k \in O} \sum_{a \in V} \sum_{c \in V} \sum_{d \in V} \frac{1}{2} {}^1T_{c,k} Y_{a,\gamma}^{1,*} Y_{i,\gamma}^{2,*} Z_{\gamma,\zeta}^* Y_{j,\zeta}^{4,*} {}^2D_{a,i,b,j} {}^2T_{a,i,d,j} V_{b,c,k,d} \quad (9390)$$

Factorized expression

$$\tau_{\gamma,\delta,w}^0 = \sum_{a \in V} {}^2D_{a,w}^1 Y_{a,\gamma}^1 Y_{a,\delta}^{1,*} \quad (3r_D r_T^2 N_v) \quad (9391)$$

$$\tau_{i,j}^1 = \sum_{a \in V} {}^1T_{a,i} f_{j,a} \quad (2N_o^2 N_v) \quad (9392)$$

$$\tau_{\gamma,i}^2 = \sum_{j \in O} Y_{j,\gamma}^2 \tau_{i,j}^1 \quad (2r_T N_o^2) \quad (9393)$$

$$\tau_{\gamma,\delta,w}^3 = \sum_{i \in O} {}^2D_{i,w}^2 Y_{i,\gamma}^{2,*} \tau_{\gamma,i}^2 \quad (3r_D r_T^2 N_o) \quad (9394)$$

$$\tau_{\gamma,\delta,w}^4 = \sum_{\epsilon \in A} Z_{\epsilon,\delta}^* \tau_{\gamma,\epsilon,w}^0 \tau_{\gamma,\epsilon,w}^3 \quad (3r_D r_T^3) \quad (9395)$$

$$\tau_{\gamma,\delta,w}^5 = \sum_{\epsilon \in A} Z_{\epsilon,\gamma} \tau_{\epsilon,\delta,w}^4 \quad (2r_D r_T^3) \quad (9396)$$

$$\tau_{\gamma,\delta,w}^6 = \sum_{i \in O} {}^2D_{i,w}^4 Y_{i,\gamma}^4 Y_{i,\delta}^{4,*} \quad (3r_D r_T^2 N_o) \quad (9397)$$

$${}^2R_{a,\gamma}^3 \leftarrow - \sum_{\delta \in A} \sum_{w \in D} \frac{1}{2} {}^2D_{a,w}^3 Y_{a,\delta}^3 \tau_{\delta,\gamma,w}^5 \tau_{\delta,\gamma,w}^6 \quad (4r_D r_T^2 N_v) \quad (9398)$$

Raw expression

$${}^2R_{b,\zeta}^3 \leftarrow - \sum_{\gamma \in A} \sum_{i \in O} \sum_{j \in O} \sum_{k \in O} \sum_{a \in V} \sum_{c \in V} \sum_{d \in V} \frac{1}{2} {}^1T_{c,k} Y_{a,\gamma}^{1,*} Y_{i,\gamma}^{2,*} Z_{\gamma,\zeta}^* Y_{j,\zeta}^{4,*} {}^2D_{a,i,b,j} {}^2T_{b,j,d,i} V_{a,c,k,d} \quad (9399)$$

Factorized expression

$$\tau^0_{\gamma,\delta,w} = \sum_{a \in V} {}^2D^1_{a,w} Y^3_{a,\gamma} Y^{1,*}_{a,\delta} \quad (3r_D r_T^2 N_v) \quad (9400)$$

$$\tau^1_{i,j} = \sum_{a \in V} {}^1T_{a,i} f_{j,a} \quad (2N_o^2 N_v) \quad (9401)$$

$$\tau^2_{\gamma,i} = \sum_{j \in O} Y^4_{j,\gamma} \tau^1_{i,j} \quad (2r_T N_o^2) \quad (9402)$$

$$\tau^3_{\gamma,\delta,w} = \sum_{i \in O} {}^2D^2_{i,w} Y^{2,*}_{i,\delta} \tau^2_{\gamma,i} \quad (3r_D r_T^2 N_o) \quad (9403)$$

$$\tau^4_{\gamma,\delta,w} = \sum_{\epsilon \in A} Z^*_{\epsilon,\delta} \tau^0_{\gamma,\epsilon,w} \tau^3_{\gamma,\epsilon,w} \quad (3r_D r_T^3) \quad (9404)$$

$$\tau^5_{\gamma,\delta,w} = \sum_{\epsilon \in A} Z_{\gamma,\epsilon} \tau^4_{\epsilon,\delta,w} \quad (2r_D r_T^3) \quad (9405)$$

$$\tau^6_{\gamma,\delta,w} = \sum_{i \in O} {}^2D^4_{i,w} Y^2_{i,\gamma} Y^{4,*}_{i,\delta} \quad (3r_D r_T^2 N_o) \quad (9406)$$

$${}^2R^3_{a,\gamma} \leftarrow - \sum_{\delta \in A} \sum_{w \in D} \frac{1}{2} {}^2D^3_{a,w} Y^1_{a,\delta} \tau^5_{\delta,\gamma,w} \tau^6_{\delta,\gamma,w} \quad (4r_D r_T^2 N_v) \quad (9407)$$

Raw expression

$${}^2R^3_{b,\zeta} \leftarrow - \sum_{\gamma \in A} \sum_{i \in O} \sum_{j \in O} \sum_{k \in O} \sum_{a \in V} \sum_{c \in V} \sum_{d \in V} \frac{1}{2} {}^1T_{c,k} Y^{1,*}_{a,\gamma} Y^{2,*}_{i,\gamma} Z^*_{\gamma,\zeta} Y^{4,*}_{j,\zeta} {}^2D^{a,i,b,j} {}^2T_{d,i,b,j} V_{a,c,k,d} \quad (9408)$$

Factorized expression

$$\tau^0_{\gamma,\delta,w} = \sum_{a \in V} {}^2D^1_{a,w} Y^1_{a,\gamma} Y^{1,*}_{a,\delta} \quad (3r_D r_T^2 N_v) \quad (9409)$$

$$\tau^1_{\gamma,\delta,w} = \sum_{i \in O} {}^2D^2_{i,w} Y^2_{i,\gamma} Y^{2,*}_{i,\delta} \quad (3r_D r_T^2 N_o) \quad (9410)$$

$$\tau^2_{\gamma,\delta,w} = \sum_{\epsilon \in A} Z^*_{\epsilon,\delta} \tau^0_{\gamma,\epsilon,w} \tau^1_{\gamma,\epsilon,w} \quad (3r_D r_T^3) \quad (9411)$$

$$\tau^3_{\gamma,\delta,w} = \sum_{\epsilon \in A} Z_{\epsilon,\gamma} \tau^2_{\epsilon,\delta,w} \quad (2r_D r_T^3) \quad (9412)$$

$$\tau^4_{i,j} = \sum_{a \in V} {}^1T_{a,i} f_{j,a} \quad (2N_o^2 N_v) \quad (9413)$$

$$\tau^5_{\gamma,i} = \sum_{j \in O} Y^4_{j,\gamma} \tau^4_{i,j} \quad (2r_T N_o^2) \quad (9414)$$

$$\tau^6_{\gamma,\delta,w} = \sum_{i \in O} {}^2D^4_{i,w} Y^{4,*}_{i,\delta} \tau^5_{\gamma,i} \quad (3r_D r_T^2 N_o) \quad (9415)$$

$${}^2R^3_{a,\gamma} \leftarrow - \sum_{\delta \in A} \sum_{w \in D} \frac{1}{2} {}^2D^3_{a,w} Y^3_{a,\delta} \tau^3_{\delta,\gamma,w} \tau^6_{\delta,\gamma,w} \quad (4r_D r_T^2 N_v) \quad (9416)$$

Raw expression

$${}^2R^3_{b,\zeta} \leftarrow - \sum_{\gamma \in A} \sum_{i \in O} \sum_{j \in O} \sum_{k \in O} \sum_{a \in V} \sum_{c \in V} \sum_{d \in V} \frac{1}{2} {}^1T_{c,k} Y^{1,*}_{a,\gamma} Y^{2,*}_{i,\gamma} Z^*_{\gamma,\zeta} Y^{4,*}_{j,\zeta} {}^2D^{a,i,b,j} {}^2T_{d,j,a,i} V_{b,c,k,d} \quad (9417)$$

Factorized expression

$$\tau^0_{i,j} = \sum_{a \in V} {}^1T_{a,i} f_{j,a} \quad (2N_o^2 N_v) \quad (9418)$$

$$\tau^1_{\gamma,i} = \sum_{j \in O} Y^2_{j,\gamma} \tau^0_{i,j} \quad (2r_T N_o^2) \quad (9419)$$

$$\tau^2_{\gamma,\delta,w} = \sum_{i \in O} {}^2D^4_{i,w} Y^{4,*}_{i,\delta} \tau^1_{\gamma,i} \quad (3r_D r_T^2 N_o) \quad (9420)$$

$$\tau^3_{\gamma,\delta,w} = \sum_{a \in V} {}^2D^1_{a,w} Y^3_{a,\gamma} Y^{1,*}_{a,\delta} \quad (3r_D r_T^2 N_v) \quad (9421)$$

$$\tau^4_{\gamma,\delta,w} = \sum_{i \in O} {}^2D^2_{i,w} Y^4_{i,\gamma} Y^{2,*}_{i,\delta} \quad (3r_D r_T^2 N_o) \quad (9422)$$

$$\tau^5_{\gamma,\delta,w} = \sum_{\epsilon \in A} Z^*_{\epsilon,\delta} \tau^3_{\gamma,\epsilon,w} \tau^4_{\gamma,\epsilon,w} \quad (3r_D r_T^3) \quad (9423)$$

$$\tau^6_{\gamma,\delta,w} = \sum_{\epsilon \in A} Z_{\gamma,\epsilon} \tau^5_{\epsilon,\delta,w} \quad (2r_D r_T^3) \quad (9424)$$

$${}^2R^3_{a,\gamma} \leftarrow - \sum_{\delta \in A} \sum_{w \in D} \frac{1}{2} {}^2D^3_{a,w} Y^1_{a,\delta} \tau^2_{\delta,\gamma,w} \tau^6_{\delta,\gamma,w} \quad (4r_D r_T^2 N_v) \quad (9425)$$

**G. Contributions from  $(H^1 T^1 T^1 T^1 T)_c$** 

Raw expression

$${}^2 R^3_{b,\zeta} \leftarrow \sum_{\gamma \in A} \sum_{i \in O} \sum_{j \in O} \sum_{k \in O} \sum_{l \in O} \sum_{a \in V} \sum_{c \in V} \sum_{d \in V} {}^1 T_{a,l} {}^1 T_{b,k} {}^1 T_{c,i} {}^1 T_{d,j} Y^{1,*}_{a,\gamma} Y^{2,*}_{i,\gamma} Z^*_{\gamma,\zeta} Y^{4,*}_{j,\zeta} {}^2 D^{a,i,b,j}_{l,c,k,d} V_{l,c,k,d} \quad (9426)$$

Factorized expression

$$\tau^0_{\alpha,i} = \sum_{a \in V} {}^1 T_{a,i} W^4_{a,\alpha} \quad (2r_V N_o N_v) \quad (9427)$$

$$\tau^1_{\gamma,\alpha,w} = \sum_{i \in O} {}^2 D^4_{i,w} Y^{4,*}_{i,\gamma} \tau^0_{\alpha,i} \quad (3r_D r_T r_V N_o) \quad (9428)$$

$$\tau^2_{\alpha,i} = \sum_{a \in V} {}^1 T_{a,i} W^2_{a,\alpha} \quad (2r_V N_o N_v) \quad (9429)$$

$$\tau^3_{\gamma,\alpha,w} = \sum_{i \in O} {}^2 D^2_{i,w} Y^{2,*}_{i,\gamma} \tau^2_{\alpha,i} \quad (3r_D r_T r_V N_o) \quad (9430)$$

$$\tau^4_{\gamma,w,i} = \sum_{a \in V} {}^2 D^1_{a,w} {}^1 T_{a,i} Y^{1,*}_{a,\gamma} \quad (3r_D r_T N_o N_v) \quad (9431)$$

$$\tau^5_{\gamma,\alpha,w} = \sum_{i \in O} W^1_{i,\alpha} \tau^4_{\gamma,w,i} \quad (2r_D r_T r_V N_o) \quad (9432)$$

$$\tau^6_{\gamma,\alpha,w} = \sum_{\beta \in B} X_{\beta,\alpha} \tau^3_{\gamma,\beta,w} \tau^5_{\gamma,\beta,w} \quad (3r_D r_T r_V^2) \quad (9433)$$

$$\tau^7_{\gamma,\alpha,w} = \sum_{\delta \in A} Z^*_{\delta,\gamma} \tau^6_{\delta,\alpha,w} \quad (2r_D r_T^2 r_V) \quad (9434)$$

$$\tau^8_{\gamma,w,i} = \sum_{\alpha \in B} W^3_{i,\alpha} \tau^1_{\gamma,\alpha,w} \tau^7_{\gamma,\alpha,w} \quad (3r_D r_T r_V N_o) \quad (9435)$$

$${}^2 R^3_{a,\gamma} \leftarrow \sum_{w \in D} \sum_{i \in O} {}^2 D^3_{a,w} {}^1 T_{a,i} \tau^8_{\gamma,w,i} \quad (3r_D r_T N_o N_v) \quad (9436)$$

**H. Contributions from  $(H^1 T^1 T^2 T)_c$** 

Raw expression

$${}^2 R^3_{b,\zeta} \leftarrow \sum_{\gamma \in A} \sum_{i \in O} \sum_{j \in O} \sum_{k \in O} \sum_{l \in O} \sum_{a \in V} \sum_{c \in V} \sum_{d \in V} \frac{1}{2} {}^1 T_{a,k} {}^1 T_{c,i} Y^{1,*}_{a,\gamma} Y^{2,*}_{i,\gamma} Z^*_{\gamma,\zeta} Y^{4,*}_{j,\zeta} {}^2 D^{a,i,b,j}_{b,j,d,l} V_{k,d,l,c} \quad (9437)$$

Factorized expression

$$\tau^0_{\gamma,\delta,w} = \sum_{i \in O} {}^2 D^4_{i,w} Y^2_{i,\gamma} Y^{4,*}_{i,\delta} \quad (3r_D r_T^2 N_o) \quad (9438)$$

$$\tau^1_{\alpha,i} = \sum_{a \in V} {}^1 T_{a,i} W^2_{a,\alpha} \quad (2r_V N_o N_v) \quad (9439)$$

$$\tau^2_{\gamma,\alpha,w} = \sum_{i \in O} {}^2 D^2_{i,w} Y^{2,*}_{i,\gamma} \tau^1_{\alpha,i} \quad (3r_D r_T r_V N_o) \quad (9440)$$

$$\tau^3_{\gamma,w,i} = \sum_{a \in V} {}^2 D^1_{a,w} {}^1 T_{a,i} Y^{1,*}_{a,\gamma} \quad (3r_D r_T N_o N_v) \quad (9441)$$

$$\tau^4_{\gamma,\alpha,w} = \sum_{i \in O} W^1_{i,\alpha} \tau^3_{\gamma,w,i} \quad (2r_D r_T r_V N_o) \quad (9442)$$

$$\tau^5_{\gamma,\alpha} = \sum_{a \in V} W^4_{a,\alpha} Y^3_{a,\gamma} \quad (2r_T r_V N_v) \quad (9443)$$

$$\tau^6_{\gamma,\alpha} = \sum_{i \in O} W^3_{i,\alpha} Y^4_{i,\gamma} \quad (2r_T r_V N_o) \quad (9444)$$

$$\tau^7_{\gamma,\alpha} = \sum_{\beta \in B} X_{\alpha,\beta} \tau^5_{\gamma,\beta} \tau^6_{\gamma,\beta} \quad (3r_T r_V^2) \quad (9445)$$

$$\tau^8_{\gamma,\alpha} = \sum_{\delta \in A} Z_{\gamma,\delta} \tau^7_{\delta,\alpha} \quad (2r_T^2 r_V) \quad (9446)$$

$$\tau^9_{\gamma,\delta,w} = \sum_{\alpha \in B} \tau^8_{\gamma,\alpha} \tau^2_{\delta,\alpha,w} \tau^4_{\delta,\alpha,w} \quad (3r_D r_T^2 r_V) \quad (9447)$$

$$\tau^{10}_{\gamma,\delta,w} = \sum_{\epsilon \in A} Z^*_{\epsilon,\delta} \tau^9_{\gamma,\epsilon,w} \quad (2r_D r_T^3) \quad (9448)$$

$${}^2 R^3_{a,\gamma} \leftarrow - \sum_{\delta \in A} \sum_{w \in D} {}^2 D^3_{a,w} Y^1_{a,\delta} \tau^0_{\delta,\gamma,w} \tau^{10}_{\delta,\gamma,w} \quad (4r_D r_T^2 N_v) \quad (9449)$$

Raw expression

$${}^2R^3_{b,\zeta} \leftarrow \sum_{\gamma \in A} \sum_{i \in O} \sum_{j \in O} \sum_{k \in O} \sum_{l \in O} \sum_{a \in V} \sum_{c \in V} \sum_{d \in V} \frac{1}{2} \quad (9450)$$

$${}^1T_{a,k} \quad {}^1T_{c,i} \quad Y^{1,*}_{a,\gamma} \quad Y^{2,*}_{i,\gamma} \quad Z^*_{\gamma,\zeta}$$

$$Y^{4,*}_{j,\zeta} \quad {}^2D^{a,i,b,j} \quad {}^2T_{b,l,d,j} \quad V_{k,c,l,d}$$

Factorized expression

$$\tau^0_{\gamma,\delta,w} = \sum_{i \in O} {}^2D^4_{i,w} Y^4_{i,\gamma} Y^{4,*}_{i,\delta} \quad (3r_D r_T^2 N_o) \quad (9451)$$

$$\tau^1_{\alpha,i} = \sum_{a \in V} {}^1T_{a,i} W^2_{a,\alpha} \quad (2r_V N_o N_v) \quad (9452)$$

$$\tau^2_{\gamma,\alpha,w} = \sum_{i \in O} {}^2D^2_{i,w} Y^{2,*}_{i,\gamma} \tau^1_{\alpha,i} \quad (3r_D r_T r_V N_o) \quad (9453)$$

$$\tau^3_{\gamma,w,i} = \sum_{a \in V} {}^2D^1_{a,w} {}^1T_{a,i} Y^{1,*}_{a,\gamma} \quad (3r_D r_T N_o N_v) \quad (9454)$$

$$\tau^4_{\gamma,\alpha,w} = \sum_{i \in O} W^1_{i,\alpha} \tau^3_{\gamma,w,i} \quad (2r_D r_T r_V N_o) \quad (9455)$$

$$\tau^5_{\gamma,\alpha} = \sum_{a \in V} W^4_{a,\alpha} Y^1_{a,\gamma} \quad (2r_T r_V N_v) \quad (9456)$$

$$\tau^6_{\gamma,\alpha} = \sum_{i \in O} W^3_{i,\alpha} Y^2_{i,\gamma} \quad (2r_T r_V N_o) \quad (9457)$$

$$\tau^7_{\gamma,\alpha} = \sum_{\beta \in B} X_{\alpha,\beta} \tau^5_{\gamma,\beta} \tau^6_{\gamma,\beta} \quad (3r_T r_V^2) \quad (9458)$$

$$\tau^8_{\gamma,\alpha} = \sum_{\delta \in A} Z_{\delta,\gamma} \tau^7_{\delta,\alpha} \quad (2r_T^2 r_V) \quad (9459)$$

$$\tau^9_{\gamma,\delta,w} = \sum_{\alpha \in B} \tau^8_{\gamma,\alpha} \tau^2_{\delta,\alpha,w} \tau^4_{\delta,\alpha,w} \quad (3r_D r_T^2 r_V) \quad (9460)$$

$$\tau^{10}_{\gamma,\delta,w} = \sum_{\epsilon \in A} Z^*_{\epsilon,\delta} \tau^9_{\gamma,\epsilon,w} \quad (2r_D r_T^3) \quad (9461)$$

$${}^2R^3_{a,\gamma} \leftarrow - \sum_{\delta \in A} \sum_{w \in D} {}^2D^3_{a,w} Y^3_{a,\delta} \tau^0_{\delta,\gamma,w} \tau^{10}_{\delta,\gamma,w} \quad (4r_D r_T^2 N_v^3) R^3_{a,\gamma} \leftarrow - \sum_{\delta \in A} \sum_{w \in D} {}^2D^3_{a,w} Y^1_{a,\delta} \tau^0_{\delta,\gamma,w} \tau^{10}_{\delta,\gamma,w} \quad (4r_D r_T^2 N_v) \quad (9462)$$

Raw expression

$${}^2R^3_{b,\zeta} \leftarrow \sum_{\gamma \in A} \sum_{i \in O} \sum_{j \in O} \sum_{k \in O} \sum_{l \in O} \sum_{a \in V} \sum_{c \in V} \sum_{d \in V} \frac{1}{2} \quad (9463)$$

$${}^1T_{a,k} \quad {}^1T_{c,i} \quad Y^{1,*}_{a,\gamma} \quad Y^{2,*}_{i,\gamma} \quad Z^*_{\gamma,\zeta}$$

$$Y^{4,*}_{j,\zeta} \quad {}^2D^{a,i,b,j} \quad {}^2T_{d,j,b,l} \quad V_{k,c,l,d}$$

Factorized expression

$$\tau^0_{\gamma,\delta,w} = \sum_{i \in O} {}^2D^4_{i,w} Y^2_{i,\gamma} Y^{4,*}_{i,\delta} \quad (3r_D r_T^2 N_o) \quad (9464)$$

$$\tau^1_{\gamma,\delta,w} = \sum_{i \in O} {}^2D^2_{i,w} Y^4_{i,\gamma} Y^{2,*}_{i,\delta} \quad (3r_D r_T^2 N_o) \quad (9465)$$

$$\tau^2_{\gamma,w,i} = \sum_{a \in V} {}^2D^1_{a,w} {}^1T_{a,i} Y^{1,*}_{a,\gamma} \quad (3r_D r_T N_o N_v) \quad (9466)$$

$$\tau^3_{\alpha,i} = \sum_{a \in V} {}^1T_{a,i} W^4_{a,\alpha} \quad (2r_V N_o N_v) \quad (9467)$$

$$\tau^4_{\alpha} = \sum_{i \in O} W^3_{i,\alpha} \tau^3_{\alpha,i} \quad (2r_V N_o) \quad (9468)$$

$$\tau^5_{\alpha} = \sum_{\beta \in B} \tau^4_{\beta} X_{\alpha,\beta} \quad (2r_V^2) \quad (9469)$$

$$\tau^6_{i,a} = \sum_{\alpha \in B} \tau^5_{\alpha} W^1_{i,\alpha} W^2_{a,\alpha} \quad (3r_V N_o N_v) \quad (9470)$$

$$\tau^7_{\gamma,i} = \sum_{a \in V} Y^3_{a,\gamma} \tau^6_{i,a} \quad (2r_T N_o N_v) \quad (9471)$$

$$\tau^8_{\gamma,\delta,w} = \sum_{i \in O} \tau^7_{\gamma,i} \tau^2_{\delta,w,i} \quad (2r_D r_T^2 N_o) \quad (9472)$$

$$\tau^9_{\gamma,\delta,w} = \sum_{\epsilon \in A} Z^*_{\epsilon,\delta} \tau^1_{\gamma,\epsilon,w} \tau^8_{\gamma,\epsilon,w} \quad (3r_D r_T^3) \quad (9473)$$

$$\tau^{10}_{\gamma,\delta,w} = \sum_{\epsilon \in A} Z_{\gamma,\epsilon} \tau^9_{\epsilon,\delta,w} \quad (2r_D r_T^3) \quad (9474)$$

$${}^2R^3_{a,\gamma} \leftarrow - \sum_{\delta \in A} \sum_{w \in D} {}^2D^3_{a,w} Y^1_{a,\delta} \tau^0_{\delta,\gamma,w} \tau^{10}_{\delta,\gamma,w} \quad (4r_D r_T^2 N_v) \quad (9475)$$

Raw expression

$${}^2R^3_{b,\zeta} \leftarrow \sum_{\gamma \in A} \sum_{i \in O} \sum_{j \in O} \sum_{k \in O} \sum_{l \in O} \sum_{a \in V} \sum_{c \in V} \sum_{d \in V} \frac{1}{2} \quad (9476)$$

$${}^1T_{a,k} \quad {}^1T_{c,i} \quad Y^{1,*}_{a,\gamma} \quad Y^{2,*}_{i,\gamma} \quad Z^*_{\gamma,\zeta}$$

$$Y^{4,*}_{j,\zeta} \quad {}^2D^{a,i,b,j} \quad {}^2T_{d,l,b,j} \quad V_{k,d,l,c}$$

Factorized expression

$$\tau^0_{\gamma,\delta,w} = \sum_{i \in O} {}^2D^4_{i,w} Y^4_{i,\gamma} Y^{4,*}_{i,\delta} \quad (3r_D r_T^2 N_o) \quad (9477)$$

$$\tau^1_{\gamma,\delta,w} = \sum_{i \in O} {}^2D^2_{i,w} Y^2_{i,\gamma} Y^{2,*}_{i,\delta} \quad (3r_D r_T^2 N_o) \quad (9478)$$

$$\tau^2_{\gamma,w,i} = \sum_{a \in V} {}^2D^1_{a,w} {}^1T_{a,i} Y^{1,*}_{a,\gamma} \quad (3r_D r_T N_o N_v) \quad (9479)$$

$$\tau^3_{\alpha,i} = \sum_{a \in V} {}^1T_{a,i} W^4_{a,\alpha} \quad (2r_V N_o N_v) \quad (9480)$$

$$\tau^4_{\alpha} = \sum_{i \in O} W^3_{i,\alpha} \tau^3_{\alpha,i} \quad (2r_V N_o) \quad (9481)$$

$$\tau^5_{\alpha} = \sum_{\beta \in B} \tau^4_{\beta} X_{\alpha,\beta} \quad (2r_V^2) \quad (9482)$$

$$\tau^6_{i,a} = \sum_{\alpha \in B} \tau^5_{\alpha} W^1_{i,\alpha} W^2_{a,\alpha} \quad (3r_V N_o N_v) \quad (9483)$$

$$\tau^7_{\gamma,i} = \sum_{a \in V} Y^1_{a,\gamma} \tau^6_{i,a} \quad (2r_T N_o N_v) \quad (9484)$$

$$\tau^8_{\gamma,\delta,w} = \sum_{i \in O} \tau^7_{\gamma,i} \tau^2_{\delta,w,i} \quad (2r_D r_T^2 N_o) \quad (9485)$$

$$\tau^9_{\gamma,\delta,w} = \sum_{\epsilon \in A} Z^*_{\epsilon,\delta} \tau^1_{\gamma,\epsilon,w} \tau^8_{\gamma,\epsilon,w} \quad (3r_D r_T^3) \quad (9486)$$

$$\tau^{10}_{\gamma,\delta,w} = \sum_{\epsilon \in A} Z_{\epsilon,\gamma} \tau^9_{\epsilon,\delta,w} \quad (2r_D r_T^3) \quad (9487)$$

$${}^2R^3_{a,\gamma} \leftarrow - \sum_{\delta \in A} \sum_{w \in D} {}^2D^3_{a,w} Y^3_{a,\delta} \tau^0_{\delta,\gamma,w} \tau^{10}_{\delta,\gamma,w} \quad (4r_D r_T^2 N_v^2) R^3_{a,\gamma} \leftarrow - \sum_{w \in D} \sum_{i \in O} {}^2D^3_{a,w} {}^1T_{a,i} \tau^{10}_{\gamma,w,i} \quad (3r_D r_T N_o N_v) \quad (9488)$$

Raw expression

$${}^2R^3_{b,\zeta} \leftarrow \sum_{\gamma \in A} \sum_{i \in O} \sum_{j \in O} \sum_{k \in O} \sum_{l \in O} \sum_{a \in V} \sum_{c \in V} \sum_{d \in V} \frac{1}{2} \quad (9489)$$

$${}^1T_{a,k} \quad {}^1T_{c,j} \quad Y^{1,*}_{a,\gamma} \quad Y^{2,*}_{i,\gamma} \quad Z^*_{\gamma,\zeta}$$

$$Y^{4,*}_{j,\zeta} \quad {}^2D^{a,i,b,j} \quad {}^2T_{b,l,d,i} \quad V_{k,d,l,c}$$

Factorized expression

$$\tau^0_{\alpha,i} = \sum_{a \in V} {}^1T_{a,i} W^2_{a,\alpha} \quad (2r_V N_o N_v) \quad (9490)$$

$$\tau^1_{\gamma,\alpha,w} = \sum_{i \in O} {}^2D^4_{i,w} Y^{4,*}_{i,\gamma} \tau^0_{\alpha,i} \quad (3r_D r_T r_V N_o) \quad (9491)$$

$$\tau^2_{\gamma,\alpha} = \sum_{a \in V} W^4_{a,\alpha} Y^3_{a,\gamma} \quad (2r_T r_V N_v) \quad (9492)$$

$$\tau^3_{\gamma,\alpha} = \sum_{i \in O} W^3_{i,\alpha} Y^4_{i,\gamma} \quad (2r_T r_V N_o) \quad (9493)$$

$$\tau^4_{\gamma,\alpha} = \sum_{\beta \in B} X_{\alpha,\beta} \tau^2_{\gamma,\beta} \tau^3_{\gamma,\beta} \quad (3r_T r_V^2) \quad (9494)$$

$$\tau^5_{\gamma,\alpha} = \sum_{\delta \in A} Z_{\gamma,\delta} \tau^4_{\delta,\alpha} \quad (2r_T^2 r_V) \quad (9495)$$

$$\tau^6_{\gamma,\delta,w} = \sum_{a \in V} {}^2D^1_{a,w} Y^1_{a,\gamma} Y^{1,*}_{a,\delta} \quad (3r_D r_T^2 N_v) \quad (9496)$$

$$\tau^7_{\gamma,\delta,w} = \sum_{i \in O} {}^2D^2_{i,w} Y^2_{i,\gamma} Y^{2,*}_{i,\delta} \quad (3r_D r_T^2 N_o) \quad (9497)$$

$$\tau^8_{\gamma,\delta,w} = \sum_{\epsilon \in A} Z^*_{\epsilon,\delta} \tau^6_{\gamma,\epsilon,w} \tau^7_{\gamma,\epsilon,w} \quad (3r_D r_T^3) \quad (9498)$$

$$\tau^9_{\gamma,\alpha,w} = \sum_{\delta \in A} \tau^5_{\delta,\alpha} \tau^8_{\delta,\gamma,w} \quad (2r_D r_T^2 r_V) \quad (9499)$$

$$\tau^{10}_{\gamma,w,i} = \sum_{\alpha \in B} W^1_{i,\alpha} \tau^1_{\gamma,\alpha,w} \tau^9_{\gamma,\alpha,w} \quad (3r_D r_T r_V N_o) \quad (9500)$$

$${}^2R^3_{a,\gamma} \leftarrow - \sum_{w \in D} \sum_{i \in O} {}^2D^3_{a,w} {}^1T_{a,i} \tau^{10}_{\gamma,w,i} \quad (3r_D r_T N_o N_v) \quad (9501)$$

Raw expression

$${}^2R^3_{b,\zeta} \leftarrow \sum_{\gamma \in A} \sum_{i \in O} \sum_{j \in O} \sum_{k \in O} \sum_{l \in O} \sum_{a \in V} \sum_{c \in V} \sum_{d \in V} \frac{1}{2} \quad (9502)$$

$${}^1T_{a,k} \quad {}^1T_{c,j} \quad Y^{1,*}_{a,\gamma} \quad Y^{2,*}_{i,\gamma} \quad Z^*_{\gamma,\zeta}$$

$$Y^{4,*}_{j,\zeta} \quad {}^2D^{a,i,b,j} \quad {}^2T_{d,i,b,l} \quad V_{k,d,l,c}$$

Factorized expression

$$\tau^0_{\alpha,i} = \sum_{a \in V} {}^1T_{a,i} W^2_{a,\alpha} \quad (2r_V N_o N_v) \quad (9503)$$

$$\tau^1_{\gamma,\alpha,w} = \sum_{i \in O} {}^2D^4_{i,w} Y^{4,*}_{i,\gamma} \tau^0_{\alpha,i} \quad (3r_D r_T r_V N_o) \quad (9504)$$

$$\tau^2_{\gamma,\delta,w} = \sum_{a \in V} {}^2D^1_{a,w} Y^3_{a,\gamma} Y^{1,*}_{a,\delta} \quad (3r_D r_T^2 N_v) \quad (9505)$$

$$\tau^3_{\gamma,\delta,w} = \sum_{i \in O} {}^2D^2_{i,w} Y^4_{i,\gamma} Y^{2,*}_{i,\delta} \quad (3r_D r_T^2 N_o) \quad (9506)$$

$$\tau^4_{\gamma,\delta,w} = \sum_{\epsilon \in A} Z^*_{\epsilon,\delta} \tau^2_{\gamma,\epsilon,w} \tau^3_{\gamma,\epsilon,w} \quad (3r_D r_T^3) \quad (9507)$$

$$\tau^5_{\gamma,\alpha} = \sum_{a \in V} W^4_{a,\alpha} Y^1_{a,\gamma} \quad (2r_T r_V N_v) \quad (9508)$$

$$\tau^6_{\gamma,\alpha} = \sum_{i \in O} W^3_{i,\alpha} Y^2_{i,\gamma} \quad (2r_T r_V N_o) \quad (9509)$$

$$\tau^7_{\gamma,\alpha} = \sum_{\beta \in B} X_{\alpha,\beta} \tau^5_{\gamma,\beta} \tau^6_{\gamma,\beta} \quad (3r_T r_V^2) \quad (9510)$$

$$\tau^8_{\gamma,\alpha} = \sum_{\delta \in A} Z_{\delta,\gamma} \tau^7_{\delta,\alpha} \quad (2r_T^2 r_V) \quad (9511)$$

$$\tau^9_{\gamma,\alpha,w} = \sum_{\delta \in A} \tau^8_{\delta,\alpha} \tau^4_{\delta,\gamma,w} \quad (2r_D r_T^2 r_V) \quad (9512)$$

$$\tau^{10}_{\gamma,w,i} = \sum_{\alpha \in B} W^1_{i,\alpha} \tau^1_{\gamma,\alpha,w} \tau^9_{\gamma,\alpha,w} \quad (3r_D r_T r_V N_o) \quad (9513)$$

$${}^2R^3_{a,\gamma} \leftarrow - \sum_{w \in D} \sum_{i \in O} {}^2D^3_{a,w} {}^1T_{a,i} \tau^{10}_{\gamma,w,i} \quad (3r_D r_T N_o N_v) \quad (9514)$$

Raw expression

$${}^2R^3_{b,\zeta} \leftarrow \sum_{\gamma \in A} \sum_{i \in O} \sum_{j \in O} \sum_{k \in O} \sum_{l \in O} \sum_{a \in V} \sum_{c \in V} \sum_{d \in V} \frac{1}{2} \quad (9515)$$

$${}^1T_{a,k} \quad {}^1T_{c,l} \quad Y^{1,*}_{a,\gamma} \quad Y^{2,*}_{i,\gamma} \quad Z^*_{\gamma,\zeta}$$

$$Y^{4,*}_{j,\zeta} \quad {}^2D^{a,i,b,j} \quad {}^2T_{b,j,d,i} \quad V_{k,c,l,d}$$

Factorized expression

$$\tau^0_{\gamma,\delta,w} = \sum_{i \in O} {}^2D^4_{i,w} Y^4_{i,\gamma} Y^{4,*}_{i,\delta} \quad (3r_D r_T^2 N_o) \quad (9516)$$

$$\tau^1_{\gamma,\delta,w} = \sum_{a \in V} {}^2D^1_{a,w} Y^1_{a,\gamma} Y^{1,*}_{a,\delta} \quad (3r_D r_T^2 N_v) \quad (9517)$$

$$\tau^2_{\gamma,\delta,w} = \sum_{i \in O} {}^2D^2_{i,w} Y^2_{i,\gamma} Y^{2,*}_{i,\delta} \quad (3r_D r_T^2 N_o) \quad (9518)$$

$$\tau^3_{\gamma,\delta,w} = \sum_{\epsilon \in A} Z^*_{\epsilon,\delta} \tau^1_{\gamma,\epsilon,w} \tau^2_{\gamma,\epsilon,w} \quad (3r_D r_T^3) \quad (9519)$$

$$\tau^4_{\gamma,\delta,w} = \sum_{\epsilon \in A} Z_{\epsilon,\gamma} \tau^3_{\epsilon,\delta,w} \quad (2r_D r_T^3) \quad (9520)$$

$$\tau^5_{\alpha,i} = \sum_{a \in V} {}^1T_{a,i} W^4_{a,\alpha} \quad (2r_V N_o N_v) \quad (9521)$$

$$\tau^6_{\alpha} = \sum_{i \in O} W^3_{i,\alpha} \tau^5_{\alpha,i} \quad (2r_V N_o) \quad (9522)$$

$$\tau^7_{\alpha} = \sum_{\beta \in B} \tau^6_{\beta} X_{\alpha,\beta} \quad (2r_V^2) \quad (9523)$$

$$\tau^8_{i,a} = \sum_{\alpha \in B} \tau^7_{\alpha} W^1_{i,\alpha} W^2_{a,\alpha} \quad (3r_V N_o N_v) \quad (9524)$$

$$\tau^9_{\gamma,i} = \sum_{a \in V} Y^3_{a,\gamma} \tau^8_{i,a} \quad (2r_T N_o N_v) \quad (9525)$$

$$\tau^{10}_{\gamma,w,i} = \sum_{\delta \in A} \tau^9_{\delta,i} \tau^0_{\delta,\gamma,w} \tau^4_{\delta,\gamma,w} \quad (3r_D r_T^2 N_o) \quad (9526)$$

$${}^2R^3_{a,\gamma} \leftarrow - \sum_{w \in D} \sum_{i \in O} {}^2D^3_{a,w} {}^1T_{a,i} \tau^{10}_{\gamma,w,i} \quad (3r_D r_T N_o N_v) \quad (9527)$$

Raw expression

$${}^2R^3_{b,\zeta} \leftarrow \sum_{\gamma \in A} \sum_{i \in O} \sum_{j \in O} \sum_{k \in O} \sum_{l \in O} \sum_{a \in V} \sum_{c \in V} \sum_{d \in V} \frac{1}{2} \quad (9528)$$

$${}^1T_{a,k} \quad {}^1T_{c,l} \quad Y^{1,*}_{a,\gamma} \quad Y^{2,*}_{i,\gamma} \quad Z^*_{\gamma,\zeta}$$

$$Y^{4,*}_{j,\zeta} \quad {}^2D^{a,i,b,j} \quad {}^2T_{d,i,b,j} \quad V_{k,c,l,d}$$

Factorized expression

$$\tau^0_{\gamma,\delta,w} = \sum_{i \in O} {}^2D^4_{i,w} Y^2_{i,\gamma} Y^{4,*}_{i,\delta} \quad (3r_D r_T^2 N_o) \quad (9529)$$

$$\tau^1_{\gamma,\delta,w} = \sum_{a \in V} {}^2D^1_{a,w} Y^3_{a,\gamma} Y^{1,*}_{a,\delta} \quad (3r_D r_T^2 N_v) \quad (9530)$$

$$\tau^2_{\gamma,\delta,w} = \sum_{i \in O} {}^2D^2_{i,w} Y^4_{i,\gamma} Y^{2,*}_{i,\delta} \quad (3r_D r_T^2 N_o) \quad (9531)$$

$$\tau^3_{\gamma,\delta,w} = \sum_{\epsilon \in A} Z^*_{\epsilon,\delta} \tau^1_{\gamma,\epsilon,w} \tau^2_{\gamma,\epsilon,w} \quad (3r_D r_T^3) \quad (9532)$$

$$\tau^4_{\gamma,\delta,w} = \sum_{\epsilon \in A} Z_{\gamma,\epsilon} \tau^3_{\epsilon,\delta,w} \quad (2r_D r_T^3) \quad (9533)$$

$$\tau^5_{\alpha,i} = \sum_{a \in V} {}^1T_{a,i} W^4_{a,\alpha} \quad (2r_V N_o N_v) \quad (9534)$$

$$\tau^6_{\alpha} = \sum_{i \in O} W^3_{i,\alpha} \tau^5_{\alpha,i} \quad (2r_V N_o) \quad (9535)$$

$$\tau^7_{\alpha} = \sum_{\beta \in B} \tau^6_{\beta} X_{\alpha,\beta} \quad (2r_V^2) \quad (9536)$$

$$\tau^8_{i,a} = \sum_{\alpha \in B} \tau^7_{\alpha} W^1_{i,\alpha} W^2_{a,\alpha} \quad (3r_V N_o N_v) \quad (9537)$$

$$\tau^9_{\gamma,i} = \sum_{a \in V} Y^1_{a,\gamma} \tau^8_{i,a} \quad (2r_T N_o N_v) \quad (9538)$$

$$\tau^{10}_{\gamma,w,i} = \sum_{\delta \in A} \tau^9_{\delta,i} \tau^0_{\delta,\gamma,w} \tau^4_{\delta,\gamma,w} \quad (3r_D r_T^2 N_o) \quad (9539)$$

$${}^2R^3_{a,\gamma} \leftarrow - \sum_{w \in D} \sum_{i \in O} {}^2D^3_{a,w} {}^1T_{a,i} \tau^{10}_{\gamma,w,i} \quad (3r_D r_T N_o N_v) \quad (9540)$$

Raw expression

$${}^2R^3_{b,\zeta} \leftarrow \sum_{\gamma \in A} \sum_{i \in O} \sum_{j \in O} \sum_{k \in O} \sum_{l \in O} \sum_{a \in V} \sum_{c \in V} \sum_{d \in V} \frac{1}{2} \quad (9541)$$

$${}^1T_{a,l} \quad {}^1T_{b,k} \quad Y^{1,*}_{a,\gamma} \quad Y^{2,*}_{i,\gamma} \quad Z^*_{\gamma,\zeta}$$

$$Y^{4,*}_{j,\zeta} \quad {}^2D^{a,i,b,j} \quad {}^2T_{c,i,d,j} \quad V_{l,c,k,d}$$

Factorized expression

$$\tau^0_{\gamma,\delta,w} = \sum_{i \in O} {}^2D^4_{i,w} Y^4_{i,\gamma} Y^{4,*}_{i,\delta} \quad (3r_D r_T^2 N_o) \quad (9542)$$

$$\tau^1_{\gamma,\delta,w} = \sum_{a \in V} {}^2D^1_{a,w} Y^1_{a,\gamma} Y^{1,*}_{a,\delta} \quad (3r_D r_T^2 N_v) \quad (9543)$$

$$\tau^2_{\alpha,i} = \sum_{a \in V} {}^1T_{a,i} W^2_{a,\alpha} \quad (2r_V N_o N_v) \quad (9544)$$

$$\tau^3_{\alpha} = \sum_{i \in O} W^1_{i,\alpha} \tau^2_{\alpha,i} \quad (2r_V N_o) \quad (9545)$$

$$\tau^4_{\alpha} = \sum_{\beta \in B} \tau^3_{\beta} X_{\beta,\alpha} \quad (2r_V^2) \quad (9546)$$

$$\tau^5_{i,a} = \sum_{\alpha \in B} \tau^4_{\alpha} W^3_{i,\alpha} W^4_{a,\alpha} \quad (3r_V N_o N_v) \quad (9547)$$

$$\tau^6_{i,j} = \sum_{a \in V} {}^1T_{a,i} \tau^5_{j,a} \quad (2N_o^2 N_v) \quad (9548)$$

$$\tau^7_{\gamma,i} = \sum_{j \in O} Y^2_{j,\gamma} \tau^6_{i,j} \quad (2r_T N_o^2) \quad (9549)$$

$$\tau^8_{\gamma,\delta,w} = \sum_{i \in O} {}^2D^2_{i,w} Y^{2,*}_{i,\delta} \tau^7_{\gamma,i} \quad (3r_D r_T^2 N_o) \quad (9550)$$

$$\tau^9_{\gamma,\delta,w} = \sum_{\epsilon \in A} Z^*_{\epsilon,\delta} \tau^1_{\gamma,\epsilon,w} \tau^8_{\gamma,\epsilon,w} \quad (3r_D r_T^3) \quad (9551)$$

$$\tau^{10}_{\gamma,\delta,w} = \sum_{\epsilon \in A} Z_{\epsilon,\gamma} \tau^9_{\epsilon,\delta,w} \quad (2r_D r_T^3) \quad (9552)$$

$${}^2R^3_{a,\gamma} \leftarrow - \sum_{\delta \in A} \sum_{w \in D} {}^2D^3_{a,w} Y^3_{a,\delta} \tau^0_{\delta,\gamma,w} \tau^{10}_{\delta,\gamma,w} \quad (4r_D r_T^2 N_v) \quad (9553)$$

Raw expression

$${}^2R^3_{b,\zeta} \leftarrow \sum_{\gamma \in A} \sum_{i \in O} \sum_{j \in O} \sum_{k \in O} \sum_{l \in O} \sum_{a \in V} \sum_{c \in V} \sum_{d \in V} \frac{1}{2} \quad (9554)$$

$${}^1T_{a,l} \quad {}^1T_{b,k} \quad Y^{1,*}_{a,\gamma} \quad Y^{2,*}_{i,\gamma} \quad Z^*_{\gamma,\zeta}$$

$$Y^{4,*}_{j,\zeta} \quad {}^2D^{a,i,b,j} \quad {}^2T_{c,j,d,i} \quad V_{l,d,k,c}$$

Factorized expression

$$\tau^0_{\alpha,i} = \sum_{a \in V} {}^1T_{a,i} W^2_{a,\alpha} \quad (2r_V N_o N_v) \quad (9555)$$

$$\tau^1_{\alpha} = \sum_{i \in O} W^1_{i,\alpha} \tau^0_{\alpha,i} \quad (2r_V N_o) \quad (9556)$$

$$\tau^2_{\alpha} = \sum_{\beta \in B} \tau^1_{\beta} X_{\beta,\alpha} \quad (2r_V^2) \quad (9557)$$

$$\tau^3_{i,a} = \sum_{\alpha \in B} \tau^2_{\alpha} W^3_{i,\alpha} W^4_{a,\alpha} \quad (3r_V N_o N_v) \quad (9558)$$

$$\tau^4_{i,j} = \sum_{a \in V} {}^1T_{a,i} \tau^3_{j,a} \quad (2N_o^2 N_v) \quad (9559)$$

$$\tau^5_{\gamma,i} = \sum_{j \in O} Y^4_{j,\gamma} \tau^4_{i,j} \quad (2r_T N_o^2) \quad (9560)$$

$$\tau^6_{\gamma,\delta,w} = \sum_{i \in O} {}^2D^4_{i,w} Y^{4,*}_{i,\delta} \tau^5_{\gamma,i} \quad (3r_D r_T^2 N_o) \quad (9561)$$

$$\tau^7_{\gamma,\delta,w} = \sum_{a \in V} {}^2D^1_{a,w} Y^1_{a,\gamma} Y^{1,*}_{a,\delta} \quad (3r_D r_T^2 N_v) \quad (9562)$$

$$\tau^8_{\gamma,\delta,w} = \sum_{i \in O} {}^2D^2_{i,w} Y^2_{i,\gamma} Y^{2,*}_{i,\delta} \quad (3r_D r_T^2 N_o) \quad (9563)$$

$$\tau^9_{\gamma,\delta,w} = \sum_{\epsilon \in A} Z^*_{\epsilon,\delta} \tau^7_{\gamma,\epsilon,w} \tau^8_{\gamma,\epsilon,w} \quad (3r_D r_T^3) \quad (9564)$$

$$\tau^{10}_{\gamma,\delta,w} = \sum_{\epsilon \in A} Z_{\epsilon,\gamma} \tau^9_{\epsilon,\delta,w} \quad (2r_D r_T^3) \quad (9565)$$

$${}^2R^3_{a,\gamma} \leftarrow - \sum_{\delta \in A} \sum_{w \in D} {}^2D^3_{a,w} Y^3_{a,\delta} \tau^{10}_{\delta,\gamma,w} \tau^6_{\delta,\gamma,w} \quad (4r_D r_T^2 N_v^3) R^3_{a,\gamma} \leftarrow - \sum_{\delta \in A} \sum_{w \in D} {}^2D^3_{a,w} Y^1_{a,\delta} \tau^0_{\delta,\gamma,w} \tau^{10}_{\delta,\gamma,w} \quad (4r_D r_T^2 N_v) \quad (9566)$$

Raw expression

$${}^2R^3_{b,\zeta} \leftarrow \sum_{\gamma \in A} \sum_{i \in O} \sum_{j \in O} \sum_{k \in O} \sum_{l \in O} \sum_{a \in V} \sum_{c \in V} \sum_{d \in V} \frac{1}{2} \quad (9567)$$

$${}^1T_{b,k} \quad {}^1T_{c,i} \quad Y^{1,*}_{a,\gamma} \quad Y^{2,*}_{i,\gamma} \quad Z^*_{\gamma,\zeta}$$

$$Y^{4,*}_{j,\zeta} \quad {}^2D^{a,i,b,j} \quad {}^2T_{a,l,d,j} \quad V_{k,d,l,c}$$

Factorized expression

$$\tau^0_{\gamma,\delta,w} = \sum_{i \in O} {}^2D^4_{i,w} Y^2_{i,\gamma} Y^{4,*}_{i,\delta} \quad (3r_D r_T^2 N_o) \quad (9568)$$

$$\tau^1_{\gamma,\delta,w} = \sum_{a \in V} {}^2D^1_{a,w} Y^3_{a,\gamma} Y^{1,*}_{a,\delta} \quad (3r_D r_T^2 N_v) \quad (9569)$$

$$\tau^2_{\alpha,i} = \sum_{a \in V} {}^1T_{a,i} W^2_{a,\alpha} \quad (2r_V N_o N_v) \quad (9570)$$

$$\tau^3_{\alpha} = \sum_{i \in O} W^1_{i,\alpha} \tau^2_{\alpha,i} \quad (2r_V N_o) \quad (9571)$$

$$\tau^4_{\alpha} = \sum_{\beta \in B} \tau^3_{\beta} X_{\beta,\alpha} \quad (2r_V^2) \quad (9572)$$

$$\tau^5_{i,a} = \sum_{\alpha \in B} \tau^4_{\alpha} W^3_{i,\alpha} W^4_{a,\alpha} \quad (3r_V N_o N_v) \quad (9573)$$

$$\tau^6_{i,j} = \sum_{a \in V} {}^1T_{a,i} \tau^5_{j,a} \quad (2N_o^2 N_v) \quad (9574)$$

$$\tau^7_{\gamma,i} = \sum_{j \in O} Y^4_{j,\gamma} \tau^6_{i,j} \quad (2r_T N_o^2) \quad (9575)$$

$$\tau^8_{\gamma,\delta,w} = \sum_{i \in O} {}^2D^2_{i,w} Y^{2,*}_{i,\delta} \tau^7_{\gamma,i} \quad (3r_D r_T^2 N_o) \quad (9576)$$

$$\tau^9_{\gamma,\delta,w} = \sum_{\epsilon \in A} Z^*_{\epsilon,\delta} \tau^1_{\gamma,\epsilon,w} \tau^8_{\gamma,\epsilon,w} \quad (3r_D r_T^3) \quad (9577)$$

$$\tau^{10}_{\gamma,\delta,w} = \sum_{\epsilon \in A} Z_{\gamma,\epsilon} \tau^9_{\epsilon,\delta,w} \quad (2r_D r_T^3) \quad (9578)$$

$${}^2R^3_{a,\gamma} \leftarrow - \sum_{\delta \in A} \sum_{w \in D} {}^2D^3_{a,w} Y^1_{a,\delta} \tau^0_{\delta,\gamma,w} \tau^{10}_{\delta,\gamma,w} \quad (4r_D r_T^2 N_v) \quad (9579)$$

Raw expression



$${}^2R^3_{b,\zeta} \leftarrow \sum_{\gamma \in A} \sum_{i \in O} \sum_{j \in O} \sum_{k \in O} \sum_{l \in O} \sum_{a \in V} \sum_{c \in V} \sum_{d \in V} \frac{1}{2} \quad (9580)$$

$${}^1T_{b,k} \quad {}^1T_{c,i} \quad Y^{1,*}_{a,\gamma} \quad Y^{2,*}_{i,\gamma} \quad Z^*_{\gamma,\zeta}$$

$$Y^{4,*}_{j,\zeta} \quad {}^2D^{a,i,b,j} \quad {}^2T_{d,j,a,l} \quad V_{k,d,l,c}$$

Factorized expression

$$\tau^0_{\alpha,i} = \sum_{a \in V} {}^1T_{a,i} W^2_{a,\alpha} \quad (2r_V N_o N_v) \quad (9581)$$

$$\tau^1_{\alpha} = \sum_{i \in O} W^1_{i,\alpha} \tau^0_{\alpha,i} \quad (2r_V N_o) \quad (9582)$$

$$\tau^2_{\alpha} = \sum_{\beta \in B} \tau^1_{\beta} X_{\beta,\alpha} \quad (2r_V^2) \quad (9583)$$

$$\tau^3_{i,a} = \sum_{\alpha \in B} \tau^2_{\alpha} W^3_{i,\alpha} W^4_{a,\alpha} \quad (3r_V N_o N_v) \quad (9584)$$

$$\tau^4_{i,j} = \sum_{a \in V} {}^1T_{a,i} \tau^3_{j,a} \quad (2N_o^2 N_v) \quad (9585)$$

$$\tau^5_{\gamma,i} = \sum_{j \in O} Y^2_{j,\gamma} \tau^4_{i,j} \quad (2r_T N_o^2) \quad (9586)$$

$$\tau^6_{\gamma,\delta,w} = \sum_{i \in O} {}^2D^4_{i,w} Y^{4,*}_{i,\delta} \tau^5_{\gamma,i} \quad (3r_D r_T^2 N_o) \quad (9587)$$

$$\tau^7_{\gamma,\delta,w} = \sum_{a \in V} {}^2D^1_{a,w} Y^3_{a,\gamma} Y^{1,*}_{a,\delta} \quad (3r_D r_T^2 N_v) \quad (9588)$$

$$\tau^8_{\gamma,\delta,w} = \sum_{i \in O} {}^2D^2_{i,w} Y^4_{i,\gamma} Y^{2,*}_{i,\delta} \quad (3r_D r_T^2 N_o) \quad (9589)$$

$$\tau^9_{\gamma,\delta,w} = \sum_{\epsilon \in A} Z^*_{\epsilon,\delta} \tau^7_{\gamma,\epsilon,w} \tau^8_{\gamma,\epsilon,w} \quad (3r_D r_T^3) \quad (9590)$$

$$\tau^{10}_{\gamma,\delta,w} = \sum_{\epsilon \in A} Z_{\gamma,\epsilon} \tau^9_{\epsilon,\delta,w} \quad (2r_D r_T^3) \quad (9591)$$

$${}^2R^3_{a,\gamma} \leftarrow - \sum_{\delta \in A} \sum_{w \in D} {}^2D^3_{a,w} Y^1_{a,\delta} \tau^{10}_{\delta,\gamma,w} \tau^6_{\delta,\gamma,w} \quad (4r_D r_T^2 N_v) \quad (9592)$$

Raw expression

$${}^2R^3_{b,\zeta} \leftarrow \sum_{\gamma \in A} \sum_{i \in O} \sum_{j \in O} \sum_{k \in O} \sum_{l \in O} \sum_{a \in V} \sum_{c \in V} \sum_{d \in V} \frac{1}{2} \quad (9593)$$

$${}^1T_{b,k} \quad {}^1T_{c,j} \quad Y^{1,*}_{a,\gamma} \quad Y^{2,*}_{i,\gamma} \quad Z^*_{\gamma,\zeta}$$

$$Y^{4,*}_{j,\zeta} \quad {}^2D^{a,i,b,j} \quad {}^2T_{a,i,d,l} \quad V_{k,d,l,c}$$

Factorized expression

$$\tau^0_{\gamma,\alpha} = \sum_{i \in O} W^3_{i,\alpha} Y^2_{i,\gamma} \quad (2r_T r_V N_o) \quad (9594)$$

$$\tau^1_{\gamma,\alpha} = \sum_{a \in V} W^4_{a,\alpha} Y^3_{a,\gamma} \quad (2r_T r_V N_v) \quad (9595)$$

$$\tau^2_{\gamma,\alpha,i} = \sum_{\delta \in A} Z_{\gamma,\delta} Y^4_{i,\delta} \tau^1_{\delta,\alpha} \quad (3r_T^2 r_V N_o) \quad (9596)$$

$$\tau^3_{\alpha,i} = \sum_{a \in V} {}^1T_{a,i} W^2_{a,\alpha} \quad (2r_V N_o N_v) \quad (9597)$$

$$\tau^4_{\gamma,\alpha,w} = \sum_{i \in O} {}^2D^2_{i,w} Y^{2,*}_{i,\gamma} \tau^3_{\alpha,i} \quad (3r_D r_T r_V N_o) \quad (9598)$$

$$\tau^5_{\gamma,w,i} = \sum_{a \in V} {}^2D^1_{a,w} {}^1T_{a,i} Y^{1,*}_{a,\gamma} \quad (3r_D r_T N_o N_v) \quad (9599)$$

$$\tau^6_{\gamma,\alpha,w} = \sum_{i \in O} W^1_{i,\alpha} \tau^5_{\gamma,w,i} \quad (2r_D r_T r_V N_o) \quad (9600)$$

$$\tau^7_{\gamma,\alpha,w} = \sum_{\beta \in B} X_{\beta,\alpha} \tau^4_{\gamma,\beta,w} \tau^6_{\gamma,\beta,w} \quad (3r_D r_T r_V^2) \quad (9601)$$

$$\tau^8_{\gamma,\alpha,w} = \sum_{\delta \in A} Z^*_{\delta,\gamma} \tau^7_{\delta,\alpha,w} \quad (2r_D r_T^2 r_V) \quad (9602)$$

$$\tau^9_{\gamma,\delta,w,i} = \sum_{\alpha \in B} \tau^0_{\gamma,\alpha} \tau^2_{\gamma,\alpha,i} \tau^8_{\delta,\alpha,w} \quad (3r_D r_T^2 r_V N_o) \quad (9603)$$

$$\tau^{10}_{\gamma,\delta,w} = \sum_{i \in O} {}^2D^4_{i,w} Y^{4,*}_{i,\delta} \tau^9_{\gamma,\delta,w,i} \quad (3r_D r_T^2 N_o) \quad (9604)$$

$${}^2R^3_{a,\gamma} \leftarrow \sum_{\delta \in A} \sum_{w \in D} \frac{1}{2} {}^2D^3_{a,w} Y^1_{a,\delta} \tau^{10}_{\delta,\gamma,w} \quad (3r_D r_T^2 N_v) \quad (9605)$$

Raw expression

$${}^2R^3_{b,\zeta} \leftarrow \sum_{\gamma \in A} \sum_{i \in O} \sum_{j \in O} \sum_{k \in O} \sum_{l \in O} \sum_{a \in V} \sum_{c \in V} \sum_{d \in V} \frac{1}{2} \quad (9606)$$

$${}^1T_{b,k} {}^1T_{c,j} Y^{1,*}_{a,\gamma} Y^{2,*}_{i,\gamma} Z^*_{\gamma,\zeta}$$

$$Y^{4,*}_{j,\zeta} {}^2D^{a,i,b,j} {}^2T_{a,l,d,i} V_{k,c,l,d}$$

Factorized expression

$$\tau^0_{\gamma,\alpha} = \sum_{a \in V} W^4_{a,\alpha} Y^1_{a,\gamma} \quad (2r_T r_V N_v) \quad (9607)$$

$$\tau^1_{\gamma,\alpha,i} = \sum_{\delta \in A} Y^2_{i,\delta} Z_{\delta,\gamma} \tau^0_{\delta,\alpha} \quad (3r_T^2 r_V N_o) \quad (9608)$$

$$\tau^2_{\gamma,\alpha} = \sum_{i \in O} W^3_{i,\alpha} Y^4_{i,\gamma} \quad (2r_T r_V N_o) \quad (9609)$$

$$\tau^3_{\alpha,i} = \sum_{a \in V} {}^1T_{a,i} W^2_{a,\alpha} \quad (2r_V N_o N_v) \quad (9610)$$

$$\tau^4_{\gamma,\alpha,w} = \sum_{i \in O} {}^2D^2_{i,w} Y^{2,*}_{i,\gamma} \tau^3_{\alpha,i} \quad (3r_D r_T r_V N_o) \quad (9611)$$

$$\tau^5_{\gamma,w,i} = \sum_{a \in V} {}^2D^1_{a,w} {}^1T_{a,i} Y^{1,*}_{a,\gamma} \quad (3r_D r_T N_o N_v) \quad (9612)$$

$$\tau^6_{\gamma,\alpha,w} = \sum_{i \in O} W^1_{i,\alpha} \tau^5_{\gamma,w,i} \quad (2r_D r_T r_V N_o) \quad (9613)$$

$$\tau^7_{\gamma,\alpha,w} = \sum_{\beta \in B} X_{\beta,\alpha} \tau^4_{\gamma,\beta,w} \tau^6_{\gamma,\beta,w} \quad (3r_D r_T r_V^2) \quad (9614)$$

$$\tau^8_{\gamma,\alpha,w} = \sum_{\delta \in A} Z^*_{\delta,\gamma} \tau^7_{\delta,\alpha,w} \quad (2r_D r_T^2 r_V) \quad (9615)$$

$$\tau^9_{\gamma,\delta,w,i} = \sum_{\alpha \in B} \tau^2_{\gamma,\alpha} \tau^1_{\gamma,\alpha,i} \tau^8_{\delta,\alpha,w} \quad (3r_D r_T^2 r_V N_o) \quad (9616)$$

$$\tau^{10}_{\gamma,\delta,w} = \sum_{i \in O} {}^2D^4_{i,w} Y^{4,*}_{i,\delta} \tau^9_{\gamma,\delta,w,i} \quad (3r_D r_T^2 N_o) \quad (9617)$$

$${}^2R^3_{a,\gamma} \leftarrow \sum_{\delta \in A} \sum_{w \in D} \frac{1}{2} {}^2D^3_{a,w} Y^3_{a,\delta} \tau^{10}_{\delta,\gamma,w} \quad (3r_D r_T^2 N_v) \quad (9618)$$

Raw expression

$${}^2R^3_{b,\zeta} \leftarrow \sum_{\gamma \in A} \sum_{i \in O} \sum_{j \in O} \sum_{k \in O} \sum_{l \in O} \sum_{a \in V} \sum_{c \in V} \sum_{d \in V} \frac{1}{2} \quad (9619)$$

$${}^1T_{b,k} {}^1T_{c,j} Y^{1,*}_{a,\gamma} Y^{2,*}_{i,\gamma} Z^*_{\gamma,\zeta}$$

$$Y^{4,*}_{j,\zeta} {}^2D^{a,i,b,j} {}^2T_{d,i,a,l} V_{k,c,l,d}$$

Factorized expression

$$\tau^0_{\gamma,\delta,w} = \sum_{i \in O} {}^2D^4_{i,w} Y^2_{i,\gamma} Y^{4,*}_{i,\delta} \quad (3r_D r_T^2 N_o) \quad (9620)$$

$$\tau^1_{\gamma,w,i} = \sum_{a \in V} {}^2D^1_{a,w} {}^1T_{a,i} Y^{1,*}_{a,\gamma} \quad (3r_D r_T N_o N_v) \quad (9621)$$

$$\tau^2_{\gamma,\alpha} = \sum_{a \in V} W^2_{a,\alpha} Y^3_{a,\gamma} \quad (2r_T r_V N_v) \quad (9622)$$

$$\tau^3_{\alpha,i} = \sum_{a \in V} {}^1T_{a,i} W^4_{a,\alpha} \quad (2r_V N_o N_v) \quad (9623)$$

$$\tau^4_{\alpha,i,j} = \sum_{\beta \in B} X_{\alpha,\beta} W^3_{j,\beta} \tau^3_{\beta,i} \quad (3r_V^2 N_o^2) \quad (9624)$$

$$\tau^5_{\gamma,\alpha,i} = \sum_{j \in O} Y^4_{j,\gamma} \tau^4_{\alpha,i,j} \quad (2r_T r_V N_o^2) \quad (9625)$$

$$\tau^6_{\gamma,i,j} = \sum_{\alpha \in B} W^1_{j,\alpha} \tau^2_{\gamma,\alpha} \tau^5_{\gamma,\alpha,i} \quad (3r_T r_V N_o^2) \quad (9626)$$

$$\tau^7_{\gamma,i,j} = \sum_{\delta \in A} Z_{\gamma,\delta} \tau^6_{\delta,i,j} \quad (2r_T^2 N_o^2) \quad (9627)$$

$$\tau^8_{\gamma,\delta,w} = \sum_{i \in O} \sum_{j \in O} {}^2D^2_{i,w} Y^{2,*}_{i,\delta} \tau^1_{\delta,w,j} \tau^7_{\gamma,i,j} \quad (4r_D r_T^2 N_o^2) \quad (9628)$$

$$\tau^9_{\gamma,\delta,w} = \sum_{\epsilon \in A} Z^*_{\epsilon,\delta} \tau^8_{\gamma,\epsilon,w} \quad (2r_D r_T^3) \quad (9629)$$

$${}^2R^3_{a,\gamma} \leftarrow \sum_{\delta \in A} \sum_{w \in D} \frac{1}{2} {}^2D^3_{a,w} Y^1_{a,\delta} \tau^0_{\delta,\gamma,w} \tau^9_{\delta,\gamma,w} \quad (4r_D r_T^2 N_v) \quad (9630)$$

Raw expression

$${}^2R^3_{b,\zeta} \leftarrow \sum_{\gamma \in A} \sum_{i \in O} \sum_{j \in O} \sum_{k \in O} \sum_{l \in O} \sum_{a \in V} \sum_{c \in V} \sum_{d \in V} \frac{1}{2} \quad (9631)$$

$${}^1T_{b,k} \quad {}^1T_{c,j} \quad Y^{1,*}_{a,\gamma} \quad Y^{2,*}_{i,\gamma} \quad Z^*_{\gamma,\zeta}$$

$$Y^{4,*}_{j,\zeta} \quad {}^2D^{a,i,b,j} \quad {}^2T_{d,l,a,i} \quad V_{k,d,l,c}$$

Factorized expression

$$\tau^0_{\gamma,\delta,w} = \sum_{i \in O} {}^2D^4_{i,w} Y^4_{i,\gamma} Y^{4,*}_{i,\delta} \quad (3r_D r_T^2 N_o) \quad (9632)$$

$$\tau^1_{\gamma,w,i} = \sum_{a \in V} {}^2D^1_{a,w} {}^1T_{a,i} Y^{1,*}_{a,\gamma} \quad (3r_D r_T N_o N_v) \quad (9633)$$

$$\tau^2_{\gamma,\alpha} = \sum_{a \in V} W^2_{a,\alpha} Y^1_{a,\gamma} \quad (2r_T r_V N_v) \quad (9634)$$

$$\tau^3_{\alpha,i} = \sum_{a \in V} {}^1T_{a,i} W^4_{a,\alpha} \quad (2r_V N_o N_v) \quad (9635)$$

$$\tau^4_{\alpha,i,j} = \sum_{\beta \in B} X_{\alpha,\beta} W^3_{j,\beta} \tau^3_{\beta,i} \quad (3r_V^2 N_o^2) \quad (9636)$$

$$\tau^5_{\gamma,\alpha,i} = \sum_{j \in O} Y^2_{j,\gamma} \tau^4_{\alpha,i,j} \quad (2r_T r_V N_o^2) \quad (9637)$$

$$\tau^6_{\gamma,i,j} = \sum_{\alpha \in B} W^1_{j,\alpha} \tau^2_{\gamma,\alpha} \tau^5_{\gamma,\alpha,i} \quad (3r_T r_V N_o^2) \quad (9638)$$

$$\tau^7_{\gamma,i,j} = \sum_{\delta \in A} Z_{\delta,\gamma} \tau^6_{\delta,i,j} \quad (2r_T^2 N_o^2) \quad (9639)$$

$$\tau^8_{\gamma,\delta,w} = \sum_{i \in O} \sum_{j \in O} {}^2D^2_{i,w} Y^{2,*}_{i,\delta} \tau^1_{\delta,w,j} \tau^7_{\gamma,i,j} \quad (4r_D r_T^2 N_o^2) \quad (9640)$$

$$\tau^9_{\gamma,\delta,w} = \sum_{\epsilon \in A} Z^*_{\epsilon,\delta} \tau^8_{\gamma,\epsilon,w} \quad (2r_D r_T^3) \quad (9641)$$

$${}^2R^3_{a,\gamma} \leftarrow \sum_{\delta \in A} \sum_{w \in D} \frac{1}{2} {}^2D^3_{a,w} Y^3_{a,\delta} \tau^0_{\delta,\gamma,w} \tau^9_{\delta,\gamma,w} \quad (4r_D r_T^2 N_v) \quad (9642)$$

Raw expression

$${}^2R^3_{b,\zeta} \leftarrow \sum_{\gamma \in A} \sum_{i \in O} \sum_{j \in O} \sum_{k \in O} \sum_{l \in O} \sum_{a \in V} \sum_{c \in V} \sum_{d \in V} \frac{1}{2} \quad (9643)$$

$${}^1T_{b,k} \quad {}^1T_{c,l} \quad Y^{1,*}_{a,\gamma} \quad Y^{2,*}_{i,\gamma} \quad Z^*_{\gamma,\zeta}$$

$$Y^{4,*}_{j,\zeta} \quad {}^2D^{a,i,b,j} \quad {}^2T_{a,i,d,j} \quad V_{k,c,l,d}$$

Factorized expression

$$\tau^0_{\alpha,i} = \sum_{a \in V} {}^1T_{a,i} W^4_{a,\alpha} \quad (2r_V N_o N_v) \quad (9644)$$

$$\tau^1_{\alpha,i,j} = \sum_{\beta \in B} X_{\alpha,\beta} W^3_{j,\beta} \tau^0_{\beta,i} \quad (3r_V^2 N_o^2) \quad (9645)$$

$$\tau^2_{\gamma,\alpha,i} = \sum_{j \in O} Y^2_{j,\gamma} \tau^1_{\alpha,i,j} \quad (2r_T r_V N_o^2) \quad (9646)$$

$$\tau^3_{\gamma,w,i} = \sum_{a \in V} {}^2D^1_{a,w} {}^1T_{a,i} Y^{1,*}_{a,\gamma} \quad (3r_D r_T N_o N_v) \quad (9647)$$

$$\tau^4_{\gamma,w,i,j} = \sum_{\delta \in A} {}^2D^2_{i,w} Y^{2,*}_{i,\delta} Z^*_{\delta,\gamma} \tau^3_{\delta,w,j} \quad (4r_D r_T^2 N_o^2) \quad (9648)$$

$$\tau^5_{\gamma,\alpha,w,i} = \sum_{j \in O} W^1_{j,\alpha} \tau^4_{\gamma,w,i,j} \quad (2r_D r_T r_V N_o^2) \quad (9649)$$

$$\tau^6_{\gamma,\alpha} = \sum_{a \in V} W^2_{a,\alpha} Y^3_{a,\gamma} \quad (2r_T r_V N_v) \quad (9650)$$

$$\tau^7_{\gamma,\alpha,i} = \sum_{\delta \in A} Z_{\gamma,\delta} Y^4_{i,\delta} \tau^6_{\delta,\alpha} \quad (3r_T^2 r_V N_o) \quad (9651)$$

$$\tau^8_{\gamma,\delta,\alpha,w} = \sum_{i \in O} \tau^7_{\gamma,\alpha,i} \tau^5_{\delta,\alpha,w,i} \quad (2r_D r_T^2 r_V N_o) \quad (9652)$$

$$\tau^9_{\gamma,\delta,w,i} = \sum_{\alpha \in B} \tau^2_{\gamma,\alpha,i} \tau^8_{\gamma,\delta,\alpha,w} \quad (2r_D r_T^2 r_V N_o) \quad (9653)$$

$$\tau^{10}_{\gamma,\delta,w} = \sum_{i \in O} {}^2D^4_{i,w} Y^{4,*}_{i,\delta} \tau^9_{\gamma,\delta,w,i} \quad (3r_D r_T^2 N_o) \quad (9654)$$

$${}^2R^3_{a,\gamma} \leftarrow \sum_{\delta \in A} \sum_{w \in D} \frac{1}{2} {}^2D^3_{a,w} Y^1_{a,\delta} \tau^{10}_{\delta,\gamma,w} \quad (3r_D r_T^2 N_v) \quad (9655)$$

Raw expression

$${}^2R^3_{b,\zeta} \leftarrow \sum_{\gamma \in A} \sum_{i \in O} \sum_{j \in O} \sum_{k \in O} \sum_{l \in O} \sum_{a \in V} \sum_{c \in V} \sum_{d \in V} \frac{1}{2} \quad (9656)$$

$${}^1T_{b,k} {}^1T_{c,l} Y^{1,*}_{a,\gamma} Y^{2,*}_{i,\gamma} Z^*_{\gamma,\zeta}$$

$$Y^{4,*}_{j,\zeta} {}^2D^{a,i,b,j} {}^2T_{d,j,a,i} V_{k,c,l,d}$$

Factorized expression

$$\tau^0_{\alpha,i} = \sum_{a \in V} {}^1T_{a,i} W^4_{a,\alpha} \quad (2r_V N_o N_v) \quad (9657)$$

$$\tau^1_{\alpha,i,j} = \sum_{\beta \in B} X_{\alpha,\beta} W^3_{j,\beta} \tau^0_{\beta,i} \quad (3r_V^2 N_o^2) \quad (9658)$$

$$\tau^2_{\gamma,\alpha,i} = \sum_{j \in O} Y^4_{j,\gamma} \tau^1_{\alpha,i,j} \quad (2r_T r_V N_o^2) \quad (9659)$$

$$\tau^3_{\gamma,w,i} = \sum_{a \in V} {}^2D^1_{a,w} {}^1T_{a,i} Y^{1,*}_{a,\gamma} \quad (3r_D r_T N_o N_v) \quad (9660)$$

$$\tau^4_{\gamma,w,i,j} = \sum_{\delta \in A} {}^2D^2_{i,w} Y^{2,*}_{i,\delta} Z^*_{\delta,\gamma} \tau^3_{\delta,w,j} \quad (4r_D r_T^2 N_o^2) \quad (9661)$$

$$\tau^5_{\gamma,\alpha,w,i} = \sum_{j \in O} W^1_{j,\alpha} \tau^4_{\gamma,w,i,j} \quad (2r_D r_T r_V N_o^2) \quad (9662)$$

$$\tau^6_{\gamma,\alpha} = \sum_{a \in V} W^2_{a,\alpha} Y^1_{a,\gamma} \quad (2r_T r_V N_v) \quad (9663)$$

$$\tau^7_{\gamma,\alpha,i} = \sum_{\delta \in A} Y^2_{i,\delta} Z_{\delta,\gamma} \tau^6_{\delta,\alpha} \quad (3r_T^2 r_V N_o) \quad (9664)$$

$$\tau^8_{\gamma,\delta,\alpha,w} = \sum_{i \in O} \tau^7_{\gamma,\alpha,i} \tau^5_{\delta,\alpha,w,i} \quad (2r_D r_T^2 r_V N_o) \quad (9665)$$

$$\tau^9_{\gamma,\delta,w,i} = \sum_{\alpha \in B} \tau^2_{\gamma,\alpha,i} \tau^8_{\gamma,\delta,\alpha,w} \quad (2r_D r_T^2 r_V N_o) \quad (9666)$$

$$\tau^{10}_{\gamma,\delta,w} = \sum_{i \in O} {}^2D^4_{i,w} Y^{4,*}_{i,\delta} \tau^9_{\gamma,\delta,w,i} \quad (3r_D r_T^2 N_o) \quad (9667)$$

$${}^2R^3_{a,\gamma} \leftarrow \sum_{\delta \in A} \sum_{w \in D} \frac{1}{2} {}^2D^3_{a,w} Y^3_{a,\delta} \tau^{10}_{\delta,\gamma,w} \quad (3r_D r_T^2 N_v) \quad (9668)$$

Raw expression

$${}^2R^3_{b,\zeta} \leftarrow \sum_{\gamma \in A} \sum_{i \in O} \sum_{j \in O} \sum_{k \in O} \sum_{l \in O} \sum_{a \in V} \sum_{c \in V} \sum_{d \in V} \frac{1}{2} \quad (9669)$$

$${}^1T_{c,i} {}^1T_{d,j} Y^{1,*}_{a,\gamma} Y^{2,*}_{i,\gamma} Z^*_{\gamma,\zeta}$$

$$Y^{4,*}_{j,\zeta} {}^2D^{a,i,b,j} {}^2T_{a,k,b,l} V_{k,c,l,d}$$

Factorized expression

$$\tau^0_{\gamma,\delta,w} = \sum_{i \in O} {}^2D^4_{i,w} Y^2_{i,\gamma} Y^{4,*}_{i,\delta} \quad (3r_D r_T^2 N_o) \quad (9670)$$

$$\tau^1_{\gamma,\delta,w} = \sum_{i \in O} {}^2D^2_{i,w} Y^4_{i,\gamma} Y^{2,*}_{i,\delta} \quad (3r_D r_T^2 N_o) \quad (9671)$$

$$\tau^2_{\gamma,w,i} = \sum_{a \in V} {}^2D^1_{a,w} {}^1T_{a,i} Y^{1,*}_{a,\gamma} \quad (3r_D r_T N_o N_v) \quad (9672)$$

$$\tau^3_{\alpha,i} = \sum_{a \in V} {}^1T_{a,i} W^2_{a,\alpha} \quad (2r_V N_o N_v) \quad (9673)$$

$$\tau^4_{\alpha,\beta} = \sum_{i \in O} W^3_{i,\beta} \tau^3_{\alpha,i} \quad (2r_V^2 N_o) \quad (9674)$$

$$\tau^5_{\alpha,i} = \sum_{\beta \in B} W^1_{i,\beta} X_{\beta,\alpha} \tau^4_{\beta,\alpha} \quad (3r_V^2 N_o) \quad (9675)$$

$$\tau^6_{i,a} = \sum_{\alpha \in B} W^4_{a,\alpha} \tau^5_{\alpha,i} \quad (2r_V N_o N_v) \quad (9676)$$

$$\tau^7_{\gamma,i} = \sum_{a \in V} Y^3_{a,\gamma} \tau^6_{i,a} \quad (2r_T N_o N_v) \quad (9677)$$

$$\tau^8_{\gamma,\delta,w} = \sum_{i \in O} \tau^7_{\gamma,i} \tau^2_{\delta,w,i} \quad (2r_D r_T^2 N_o) \quad (9678)$$

$$\tau^9_{\gamma,\delta,w} = \sum_{\epsilon \in A} Z^*_{\epsilon,\delta} \tau^1_{\gamma,\epsilon,w} \tau^8_{\gamma,\epsilon,w} \quad (3r_D r_T^3) \quad (9679)$$

$$\tau^{10}_{\gamma,\delta,w} = \sum_{\epsilon \in A} Z_{\gamma,\epsilon} \tau^9_{\epsilon,\delta,w} \quad (2r_D r_T^3) \quad (9680)$$

$${}^2R^3_{a,\gamma} \leftarrow \sum_{\delta \in A} \sum_{w \in D} \frac{1}{2} {}^2D^3_{a,w} Y^1_{a,\delta} \tau^0_{\delta,\gamma,w} \tau^{10}_{\delta,\gamma,w} \quad (4r_D r_T^2 N_v) \quad (9681)$$

Raw expression

$${}^2R^3_{b,\zeta} \leftarrow \sum_{\gamma \in A} \sum_{i \in O} \sum_{j \in O} \sum_{k \in O} \sum_{l \in O} \sum_{a \in V} \sum_{c \in V} \sum_{d \in V} \frac{1}{2} \quad (9682)$$

$${}^1T_{c,i} \quad {}^1T_{d,j} \quad Y^{1,*}_{a,\gamma} \quad Y^{2,*}_{i,\gamma} \quad Z^*_{\gamma,\zeta}$$

$$Y^{4,*}_{j,\zeta} \quad {}^2D^{a,i,b,j} \quad {}^2T_{b,k,a,l} \quad V_{k,d,l,c}$$

Factorized expression

$$\tau^0_{\gamma,\delta,w} = \sum_{i \in O} {}^2D^4_{i,w} Y^4_{i,\gamma} Y^{4,*}_{i,\delta} \quad (3r_D r_T^2 N_o) \quad (9683)$$

$$\tau^1_{\gamma,\delta,w} = \sum_{i \in O} {}^2D^2_{i,w} Y^2_{i,\gamma} Y^{2,*}_{i,\delta} \quad (3r_D r_T^2 N_o) \quad (9684)$$

$$\tau^2_{\gamma,w,i} = \sum_{a \in V} {}^2D^1_{a,w} {}^1T_{a,i} Y^{1,*}_{a,\gamma} \quad (3r_D r_T N_o N_v) \quad (9685)$$

$$\tau^3_{\alpha,i} = \sum_{a \in V} {}^1T_{a,i} W^2_{a,\alpha} \quad (2r_V N_o N_v) \quad (9686)$$

$$\tau^4_{\alpha,\beta} = \sum_{i \in O} W^3_{i,\beta} \tau^3_{\alpha,i} \quad (2r_V^2 N_o) \quad (9687)$$

$$\tau^5_{\alpha,i} = \sum_{\beta \in B} W^1_{i,\beta} X_{\beta,\alpha} \tau^4_{\beta,\alpha} \quad (3r_V^2 N_o) \quad (9688)$$

$$\tau^6_{i,a} = \sum_{\alpha \in B} W^4_{a,\alpha} \tau^5_{\alpha,i} \quad (2r_V N_o N_v) \quad (9689)$$

$$\tau^7_{\gamma,i} = \sum_{a \in V} Y^1_{a,\gamma} \tau^6_{i,a} \quad (2r_T N_o N_v) \quad (9690)$$

$$\tau^8_{\gamma,\delta,w} = \sum_{i \in O} \tau^7_{\gamma,i} \tau^2_{\delta,w,i} \quad (2r_D r_T^2 N_o) \quad (9691)$$

$$\tau^9_{\gamma,\delta,w} = \sum_{\epsilon \in A} Z^*_{\epsilon,\delta} \tau^1_{\gamma,\epsilon,w} \tau^8_{\gamma,\epsilon,w} \quad (3r_D r_T^3) \quad (9692)$$

$$\tau^{10}_{\gamma,\delta,w} = \sum_{\epsilon \in A} Z_{\epsilon,\gamma} \tau^9_{\epsilon,\delta,w} \quad (2r_D r_T^3) \quad (9693)$$

$${}^2R^3_{a,\gamma} \leftarrow \sum_{\delta \in A} \sum_{w \in D} \frac{1}{2} {}^2D^3_{a,w} Y^3_{a,\delta} \tau^0_{\delta,\gamma,w} \tau^{10}_{\delta,\gamma,w} \quad (4r_D r_T^2 N_v) \quad (9694)$$

Raw expression

$${}^2R^3_{b,\zeta} \leftarrow \sum_{\gamma \in A} \sum_{i \in O} \sum_{j \in O} \sum_{k \in O} \sum_{l \in O} \sum_{a \in V} \sum_{c \in V} \sum_{d \in V} \frac{1}{2} \quad (9695)$$

$${}^1T_{c,i} \quad {}^1T_{d,k} \quad Y^{1,*}_{a,\gamma} \quad Y^{2,*}_{i,\gamma} \quad Z^*_{\gamma,\zeta}$$

$$Y^{4,*}_{j,\zeta} \quad {}^2D^{a,i,b,j} \quad {}^2T_{a,l,b,j} \quad V_{k,c,l,d}$$

Factorized expression

$$\tau^0_{\gamma,w,i} = \sum_{a \in V} {}^2D^1_{a,w} {}^1T_{a,i} Y^{1,*}_{a,\gamma} \quad (3r_D r_T N_o N_v) \quad (9696)$$

$$\tau^1_{\gamma,\alpha} = \sum_{a \in V} W^2_{a,\alpha} Y^1_{a,\gamma} \quad (2r_T r_V N_v) \quad (9697)$$

$$\tau^2_{\gamma,\alpha,i} = \sum_{\beta \in B} W^1_{i,\beta} X_{\beta,\alpha} \tau^1_{\gamma,\beta} \quad (3r_T r_V^2 N_o) \quad (9698)$$

$$\tau^3_{\gamma,\alpha} = \sum_{a \in V} W^4_{a,\alpha} Y^3_{a,\gamma} \quad (2r_T r_V N_v) \quad (9699)$$

$$\tau^4_{\gamma,\alpha,i} = \sum_{\delta \in A} Z_{\gamma,\delta} Y^4_{i,\delta} \tau^3_{\delta,\alpha} \quad (3r_T^2 r_V N_o) \quad (9700)$$

$$\tau^5_{\gamma,i,j,k} = \sum_{\alpha \in B} W^3_{j,\alpha} \tau^2_{\gamma,\alpha,i} \tau^4_{\gamma,\alpha,k} \quad (3r_T r_V N_o^3) \quad (9701)$$

$$\tau^6_{i,j,k,l} = \sum_{\gamma \in A} Y^2_{k,\gamma} \tau^5_{\gamma,i,j,l} \quad (2r_T N_o^4) \quad (9702)$$

$$\tau^7_{\gamma,w,i,j} = \sum_{k \in O} \sum_{l \in O} {}^2D^2_{k,w} Y^{2,*}_{k,\gamma} \tau^0_{\gamma,w,l} \tau^6_{l,i,k,j} \quad (4r_D r_T N_o^4) \quad (9703)$$

$$\tau^8_{\gamma,w,i} = \sum_{\delta \in A} \sum_{j \in O} {}^2D^4_{j,w} Z^*_{\delta,\gamma} Y^{4,*}_{j,\gamma} \tau^7_{\delta,w,i,j} \quad (4r_D r_T^2 N_o^2) \quad (9704)$$

$${}^2R^3_{a,\gamma} \leftarrow \sum_{w \in D} \sum_{i \in O} \frac{1}{2} {}^2D^3_{a,w} {}^1T_{a,i} \tau^8_{\gamma,w,i} \quad (3r_D r_T N_o N_v) \quad (9705)$$

Raw expression

$${}^2R^3_{b,\zeta} \leftarrow \sum_{\gamma \in A} \sum_{i \in O} \sum_{j \in O} \sum_{k \in O} \sum_{l \in O} \sum_{a \in V} \sum_{c \in V} \sum_{d \in V} \frac{1}{2} \quad (9706)$$

$${}^1T_{c,i} \quad {}^1T_{d,k} \quad Y^{1,*}_{a,\gamma} \quad Y^{2,*}_{i,\gamma} \quad Z^*_{\gamma,\zeta}$$

$$Y^{4,*}_{j,\zeta} \quad {}^2D^{a,i,b,j} \quad {}^2T_{b,j,a,l} \quad V_{k,c,l,d}$$

Factorized expression

$$\tau^0_{\gamma,w,i} = \sum_{a \in V} {}^2D^1_{a,w} {}^1T_{a,i} Y^{1,*}_{a,\gamma} \quad (3r_D r_T N_o N_v) \quad (9707)$$

$$\tau^1_{\gamma,\alpha} = \sum_{a \in V} W^4_{a,\alpha} Y^1_{a,\gamma} \quad (2r_T r_V N_v) \quad (9708)$$

$$\tau^2_{\gamma,\alpha,i} = \sum_{\beta \in B} X_{\alpha,\beta} W^3_{i,\beta} \tau^1_{\gamma,\beta} \quad (3r_T r_V^2 N_o) \quad (9709)$$

$$\tau^3_{\gamma,\alpha} = \sum_{a \in V} W^2_{a,\alpha} Y^3_{a,\gamma} \quad (2r_T r_V N_v) \quad (9710)$$

$$\tau^4_{\gamma,\alpha,i} = \sum_{\delta \in A} Z_{\gamma,\delta} Y^4_{i,\delta} \tau^3_{\delta,\alpha} \quad (3r_T^2 r_V N_o) \quad (9711)$$

$$\tau^5_{\gamma,i,j,k} = \sum_{\alpha \in B} W^1_{i,\alpha} \tau^2_{\gamma,\alpha,j} \tau^4_{\gamma,\alpha,k} \quad (3r_T r_V N_o^3) \quad (9712)$$

$$\tau^6_{i,j,k,l} = \sum_{\gamma \in A} Y^2_{k,\gamma} \tau^5_{\gamma,i,j,l} \quad (2r_T N_o^4) \quad (9713)$$

$$\tau^7_{\gamma,w,i,j} = \sum_{k \in O} \sum_{l \in O} {}^2D^2_{k,w} Y^{2,*}_{k,\gamma} \tau^0_{\gamma,w,l} \tau^6_{l,i,j,k} \quad (4r_D r_T N_o^4) \quad (9714)$$

$$\tau^8_{\gamma,w,i} = \sum_{\delta \in A} \sum_{j \in O} {}^2D^4_{j,w} Z^*_{\delta,\gamma} Y^{4,*}_{j,\gamma} \tau^7_{\delta,w,i,j} \quad (4r_D r_T^2 N_o^2) \quad (9715)$$

$${}^2R^3_{a,\gamma} \leftarrow \sum_{w \in D} \sum_{i \in O} \frac{1}{2} {}^2D^3_{a,w} {}^1T_{a,i} \tau^8_{\gamma,w,i} \quad (3r_D r_T N_o N_v) \quad (9716)$$

Raw expression

$${}^2R^3_{b,\zeta} \leftarrow \sum_{\gamma \in A} \sum_{i \in O} \sum_{j \in O} \sum_{k \in O} \sum_{l \in O} \sum_{a \in V} \sum_{c \in V} \sum_{d \in V} \frac{1}{2} {}^1T_{c,j} {}^1T_{d,k} Y^{1,*}_{a,\gamma} Y^{2,*}_{i,\gamma} Z^*_{\gamma,\zeta} Y^{4,*}_{j,\zeta} {}^2D^{a,i,b,j}_{a,i,b,l} {}^2T_{a,i,b,l} V_{k,c,l,d} \quad (9717)$$

Factorized expression

$$\tau^0_{\gamma,\alpha} = \sum_{a \in V} W^2_{a,\alpha} Y^3_{a,\gamma} \quad (2r_T r_V N_v) \quad (9718)$$

$$\tau^1_{\gamma,\alpha,i} = \sum_{\delta \in A} Z_{\gamma,\delta} Y^4_{i,\delta} \tau^0_{\delta,\alpha} \quad (3r_T^2 r_V N_o) \quad (9719)$$

$$\tau^2_{\gamma,\delta,w} = \sum_{a \in V} {}^2D^1_{a,w} Y^1_{a,\gamma} Y^{1,*}_{a,\delta} \quad (3r_D r_T^2 N_v) \quad (9720)$$

$$\tau^3_{\alpha,i} = \sum_{a \in V} {}^1T_{a,i} W^4_{a,\alpha} \quad (2r_V N_o N_v) \quad (9721)$$

$$\tau^4_{\alpha,i,j} = \sum_{\beta \in B} X_{\alpha,\beta} W^3_{j,\beta} \tau^3_{\beta,i} \quad (3r_V^2 N_o^2) \quad (9722)$$

$$\tau^5_{\gamma,\alpha,i} = \sum_{j \in O} Y^2_{j,\gamma} \tau^4_{\alpha,i,j} \quad (2r_T r_V N_o^2) \quad (9723)$$

$$\tau^6_{\gamma,\delta,\alpha,w} = \sum_{i \in O} {}^2D^2_{i,w} Y^{2,*}_{i,\delta} \tau^2_{\gamma,\delta,w} \tau^5_{\gamma,\alpha,i} \quad (4r_D r_T^2 r_V N_o) \quad (9724)$$

$$\tau^7_{\gamma,\alpha,w,i} = \sum_{\delta \in A} \tau^1_{\delta,\alpha,i} \tau^6_{\delta,\gamma,\alpha,w} \quad (2r_D r_T^2 r_V N_o) \quad (9725)$$

$$\tau^8_{\gamma,w,i,j} = \sum_{\alpha \in B} W^1_{i,\alpha} \tau^7_{\gamma,\alpha,w,j} \quad (2r_D r_T r_V N_o^2) \quad (9726)$$

$$\tau^9_{\gamma,w,i} = \sum_{\delta \in A} \sum_{j \in O} {}^2D^4_{j,w} Z^*_{\delta,\gamma} Y^{4,*}_{j,\gamma} \tau^8_{\delta,w,i,j} \quad (4r_D r_T^2 N_o^2) \quad (9727)$$

$${}^2R^3_{a,\gamma} \leftarrow \sum_{w \in D} \sum_{i \in O} \frac{1}{2} {}^2D^3_{a,w} {}^1T_{a,i} \tau^9_{\gamma,w,i} \quad (3r_D r_T N_o N_v) \quad (9728)$$

Raw expression

$${}^2R^3_{b,\zeta} \leftarrow \sum_{\gamma \in A} \sum_{i \in O} \sum_{j \in O} \sum_{k \in O} \sum_{l \in O} \sum_{a \in V} \sum_{c \in V} \sum_{d \in V} \frac{1}{2} {}^1T_{c,j} {}^1T_{d,k} Y^{1,*}_{a,\gamma} Y^{2,*}_{i,\gamma} Z^*_{\gamma,\zeta} Y^{4,*}_{j,\zeta} {}^2D^{a,i,b,j}_{a,i,b,l} {}^2T_{b,l,a,i} V_{k,c,l,d} \quad (9729)$$

Factorized expression

$$\tau^0_{\gamma,\alpha} = \sum_{a \in V} W^2_{a,\alpha} Y^1_{a,\gamma} \quad (2r_T r_V N_v) \quad (9730)$$

$$\tau^1_{\gamma,\alpha,i} = \sum_{\delta \in A} Y^2_{i,\delta} Z_{\delta,\gamma} \tau^0_{\delta,\alpha} \quad (3r_T^2 r_V N_o) \quad (9731)$$

$$\tau^1_{\gamma,\alpha,w} = \sum_{i \in O} {}^2D^4_{i,w} Y^{4,*}_{i,\gamma} \tau^0_{\alpha,i} \quad (3r_D r_T r_V N_o) \quad (9743)$$

$$\tau^2_{\gamma,\delta,w} = \sum_{a \in V} {}^2D^1_{a,w} Y^3_{a,\gamma} Y^{1,*}_{a,\delta} \quad (3r_D r_T^2 N_v) \quad (9732)$$

$$\tau^2_{\gamma,\delta,w} = \sum_{a \in V} {}^2D^1_{a,w} Y^1_{a,\gamma} Y^{1,*}_{a,\delta} \quad (3r_D r_T^2 N_v) \quad (9744)$$

$$\tau^3_{\alpha,i} = \sum_{a \in V} {}^1T_{a,i} W^4_{a,\alpha} \quad (2r_V N_o N_v) \quad (9733)$$

$$\tau^3_{\gamma,\alpha} = \sum_{i \in O} W^3_{i,\alpha} Y^2_{i,\gamma} \quad (2r_T r_V N_o) \quad (9745)$$

$$\tau^4_{\alpha,i,j} = \sum_{\beta \in B} X_{\alpha,\beta} W^3_{j,\beta} \tau^3_{\beta,i} \quad (3r_V^2 N_o^2) \quad (9734)$$

$$\tau^4_{\gamma,\alpha} = \sum_{a \in V} W^4_{a,\alpha} Y^3_{a,\gamma} \quad (2r_T r_V N_v) \quad (9746)$$

$$\tau^5_{\gamma,\alpha,i} = \sum_{j \in O} Y^4_{j,\gamma} \tau^4_{\alpha,i,j} \quad (2r_T r_V N_o^2) \quad (9735)$$

$$\tau^5_{\gamma,\alpha,i} = \sum_{\delta \in A} Z_{\gamma,\delta} Y^4_{i,\delta} \tau^4_{\delta,\alpha} \quad (3r_T^2 r_V N_o) \quad (9747)$$

$$\tau^6_{\gamma,\delta,\alpha,w} = \sum_{i \in O} {}^2D^2_{i,w} Y^{2,*}_{i,\delta} \tau^2_{\gamma,\delta,w} \tau^5_{\gamma,\alpha,i} \quad (4r_D r_T^2 r_V N_o) \quad (9736)$$

$$\tau^6_{\gamma,\alpha,w} = \sum_{\delta \in A} \sum_{i \in O} {}^2D^2_{i,w} Y^{2,*}_{i,\gamma} \tau^3_{\delta,\alpha} \tau^2_{\delta,\gamma,w} \tau^5_{\delta,\alpha,i} \quad (5r_D r_T^2 r_V N_o) \quad (9748)$$

$$\tau^7_{\gamma,\alpha,w,i} = \sum_{\delta \in A} \tau^1_{\delta,\alpha,i} \tau^6_{\delta,\gamma,\alpha,w} \quad (2r_D r_T^2 r_V N_o) \quad (9737)$$

$$\tau^7_{\gamma,\alpha,w} = \sum_{\beta \in B} X_{\alpha,\beta} \tau^6_{\gamma,\beta,w} \quad (2r_D r_T r_V^2) \quad (9749)$$

$$\tau^8_{\gamma,w,i,j} = \sum_{\alpha \in B} W^1_{i,\alpha} \tau^7_{\gamma,\alpha,w,j} \quad (2r_D r_T r_V N_o^2) \quad (9738)$$

$$\tau^8_{\gamma,\alpha,w} = \sum_{\delta \in A} Z^*_{\delta,\gamma} \tau^7_{\delta,\alpha,w} \quad (2r_D r_T^2 r_V) \quad (9750)$$

$$\tau^9_{\gamma,w,i} = \sum_{\delta \in A} \sum_{j \in O} {}^2D^4_{j,w} Z^*_{\delta,\gamma} Y^{4,*}_{j,\gamma} \tau^8_{\delta,w,i,j} \quad (4r_D r_T^2 N_o^2) \quad (9739)$$

$$\tau^9_{\gamma,w,i} = \sum_{\alpha \in B} W^1_{i,\alpha} \tau^1_{\gamma,\alpha,w} \tau^8_{\gamma,\alpha,w} \quad (3r_D r_T r_V N_o) \quad (9751)$$

$${}^2R^3_{a,\gamma} \leftarrow \sum_{w \in D} \sum_{i \in O} \frac{1}{2} {}^2D^3_{a,w} {}^1T_{a,i} \tau^9_{\gamma,w,i} \quad (3r_D r_T N_o N_v) \quad (9740)$$

$${}^2R^3_{a,\gamma} \leftarrow \sum_{w \in D} \sum_{i \in O} \frac{1}{2} {}^2D^3_{a,w} {}^1T_{a,i} \tau^9_{\gamma,w,i} \quad (3r_D r_T N_o N_v) \quad (9752)$$

Raw expression

$${}^2R^3_{b,\zeta} \leftarrow - \sum_{\gamma \in A} \sum_{i \in O} \sum_{j \in O} \sum_{k \in O} \sum_{l \in O} \sum_{a \in V} \sum_{c \in V} \sum_{d \in V} {}^1T_{a,k} \\ {}^1T_{c,i} Y^{1,*}_{a,\gamma} Y^{2,*}_{i,\gamma} Z^*_{\gamma,\zeta} Y^{4,*}_{j,\zeta} {}^2D^{a,i,b,j} {}^2T_{b,j,d,l} V_{k,c,l,d} \quad (9741)$$

Factorized expression

$$\tau^0_{\alpha,i} = \sum_{a \in V} {}^1T_{a,i} W^2_{a,\alpha} \quad (2r_V N_o N_v) \quad (9742)$$

Raw expression

$${}^2R^3_{b,\zeta} \leftarrow - \sum_{\gamma \in A} \sum_{i \in O} \sum_{j \in O} \sum_{k \in O} \sum_{l \in O} \sum_{a \in V} \sum_{c \in V} \sum_{d \in V} {}^1T_{a,k} \\ {}^1T_{c,i} Y^{1,*}_{a,\gamma} Y^{2,*}_{i,\gamma} Z^*_{\gamma,\zeta} Y^{4,*}_{j,\zeta} {}^2D^{a,i,b,j} {}^2T_{d,l,b,j} V_{k,c,l,d} \quad (9753)$$

Factorized expression

$$\tau^0_{\alpha,i} = \sum_{a \in V} {}^1T_{a,i} W^2_{a,\alpha} \quad (2r_V N_o N_v) \quad (9754)$$

$$\tau^1_{\gamma,\alpha,w} = \sum_{i \in O} {}^2D^4_{i,w} Y^{4,*}_{i,\gamma} \tau^0_{\alpha,i} \quad (3r_D r_T r_V N_o) \quad (9755)$$

$$\tau^1_{\alpha,i} = \sum_{a \in V} {}^1T_{a,i} W^4_{a,\alpha} \quad (2r_V N_o N_v) \quad (9767)$$

$$\tau^2_{\gamma,\delta,w} = \sum_{a \in V} {}^2D^1_{a,w} Y^3_{a,\gamma} Y^{1,*}_{a,\delta} \quad (3r_D r_T^2 N_v) \quad (9756)$$

$$\tau^2_{\alpha,i,j} = \sum_{\beta \in B} X_{\alpha,\beta} W^3_{j,\beta} \tau^1_{\beta,i} \quad (3r_V^2 N_o^2) \quad (9768)$$

$$\tau^3_{\gamma,\alpha} = \sum_{a \in V} W^4_{a,\alpha} Y^1_{a,\gamma} \quad (2r_T r_V N_v) \quad (9757)$$

$$\tau^3_{\gamma,\alpha,i} = \sum_{j \in O} Y^4_{j,\gamma} \tau^2_{\alpha,i,j} \quad (2r_T r_V N_o^2) \quad (9769)$$

$$\tau^4_{\gamma,\alpha,i} = \sum_{\delta \in A} Y^2_{i,\delta} Z_{\delta,\gamma} \tau^3_{\delta,\alpha} \quad (3r_T^2 r_V N_o) \quad (9758)$$

$$\tau^4_{\gamma,i,j} = \sum_{\alpha \in B} W^1_{j,\alpha} \tau^0_{\gamma,\alpha} \tau^3_{\gamma,\alpha,i} \quad (3r_T r_V N_o^2) \quad (9770)$$

$$\tau^5_{\gamma,\alpha} = \sum_{i \in O} W^3_{i,\alpha} Y^4_{i,\gamma} \quad (2r_T r_V N_o) \quad (9759)$$

$$\tau^5_{\gamma,i,j} = \sum_{\delta \in A} Z_{\gamma,\delta} \tau^4_{\delta,i,j} \quad (2r_T^2 N_o^2) \quad (9771)$$

$$\tau^6_{\gamma,\alpha,w} = \sum_{\delta \in A} \sum_{i \in O} {}^2D^2_{i,w} Y^{2,*}_{i,\gamma} \tau^5_{\delta,\alpha} \tau^2_{\delta,\gamma,w} \tau^4_{\delta,\alpha,i} \quad (5r_D r_T^2 r_V N_o) \quad (9760)$$

$$\tau^6_{\gamma,\delta,w} = \sum_{a \in V} {}^2D^1_{a,w} Y^1_{a,\gamma} Y^{1,*}_{a,\delta} \quad (3r_D r_T^2 N_v) \quad (9772)$$

$$\tau^7_{\gamma,\delta,w} = \sum_{i \in O} {}^2D^2_{i,w} Y^2_{i,\gamma} Y^{2,*}_{i,\delta} \quad (3r_D r_T^2 N_o) \quad (9773)$$

$$\tau^7_{\gamma,\alpha,w} = \sum_{\beta \in B} X_{\alpha,\beta} \tau^6_{\gamma,\beta,w} \quad (2r_D r_T r_V^2) \quad (9761)$$

$$\tau^8_{\gamma,\delta,w} = \sum_{\epsilon \in A} Z^*_{\epsilon,\delta} \tau^6_{\gamma,\epsilon,w} \tau^7_{\gamma,\epsilon,w} \quad (3r_D r_T^3) \quad (9774)$$

$$\tau^8_{\gamma,\alpha,w} = \sum_{\delta \in A} Z^*_{\delta,\gamma} \tau^7_{\delta,\alpha,w} \quad (2r_D r_T^2 r_V) \quad (9762)$$

$$\tau^9_{\gamma,w,i,j} = \sum_{\delta \in A} \tau^5_{\delta,i,j} \tau^8_{\delta,\gamma,w} \quad (2r_D r_T^2 N_o^2) \quad (9775)$$

$$\tau^9_{\gamma,w,i} = \sum_{\alpha \in B} W^1_{i,\alpha} \tau^1_{\gamma,\alpha,w} \tau^8_{\gamma,\alpha,w} \quad (3r_D r_T r_V N_o) \quad (9763)$$

$$\tau^{10}_{\gamma,w,i} = \sum_{j \in O} {}^2D^4_{j,w} Y^{4,*}_{j,\gamma} \tau^9_{\gamma,w,j,i} \quad (3r_D r_T N_o^2) \quad (9776)$$

$${}^2R^3_{a,\gamma} \leftarrow \sum_{w \in D} \sum_{i \in O} \frac{1}{2} {}^2D^3_{a,w} {}^1T_{a,i} \tau^9_{\gamma,w,i} \quad (3r_D r_T N_o N_v) \quad (9764)$$

$${}^2R^3_{a,\gamma} \leftarrow \sum_{w \in D} \sum_{i \in O} \frac{1}{2} {}^2D^3_{a,w} {}^1T_{a,i} \tau^{10}_{\gamma,w,i} \quad (3r_D r_T N_o N_v) \quad (9777)$$

Raw expression

$${}^2R^3_{b,\zeta} \leftarrow - \sum_{\gamma \in A} \sum_{i \in O} \sum_{j \in O} \sum_{k \in O} \sum_{l \in O} \sum_{a \in V} \sum_{c \in V} \sum_{d \in V} {}^1T_{a,k} \\ {}^1T_{c,l} Y^{1,*}_{a,\gamma} Y^{2,*}_{i,\gamma} Z^*_{\gamma,\zeta} \\ Y^{4,*}_{j,\zeta} {}^2D^{a,i,b,j} {}^2T_{b,j,d,i} V_{k,d,l,c} \quad (9765)$$

Raw expression

$${}^2R^3_{b,\zeta} \leftarrow - \sum_{\gamma \in A} \sum_{i \in O} \sum_{j \in O} \sum_{k \in O} \sum_{l \in O} \sum_{a \in V} \sum_{c \in V} \sum_{d \in V} {}^1T_{a,k} \\ {}^1T_{c,l} Y^{1,*}_{a,\gamma} Y^{2,*}_{i,\gamma} Z^*_{\gamma,\zeta} \\ Y^{4,*}_{j,\zeta} {}^2D^{a,i,b,j} {}^2T_{d,i,b,j} V_{k,d,l,c} \quad (9778)$$

Factorized expression

$$\tau^0_{\gamma,\alpha} = \sum_{a \in V} W^2_{a,\alpha} Y^3_{a,\gamma} \quad (2r_T r_V N_v) \quad (9766)$$

Factorized expression

$$\tau^0_{\gamma,\alpha} = \sum_{a \in V} W^2_{a,\alpha} Y^1_{a,\gamma} \quad (2r_T r_V N_v) \quad (9779)$$



$$\tau^1_{\alpha,i} = \sum_{a \in V} {}^1T_{a,i} W^4_{a,\alpha} \quad (2r_V N_o N_v) \quad (9780)$$

$$\tau^1_{\gamma,\delta,w} = \sum_{a \in V} {}^2D^1_{a,w} Y^1_{a,\gamma} Y^{1,*}_{a,\delta} \quad (3r_D r_T^2 N_v) \quad (9793)$$

$$\tau^2_{\alpha,i,j} = \sum_{\beta \in B} X_{\alpha,\beta} W^3_{j,\beta} \tau^1_{\beta,i} \quad (3r_V^2 N_o^2) \quad (9781)$$

$$\tau^2_{\gamma,\delta,w} = \sum_{i \in O} {}^2D^2_{i,w} Y^2_{i,\gamma} Y^{2,*}_{i,\delta} \quad (3r_D r_T^2 N_o) \quad (9794)$$

$$\tau^3_{\gamma,\alpha,i} = \sum_{j \in O} Y^2_{j,\gamma} \tau^2_{\alpha,i,j} \quad (2r_T r_V N_o^2) \quad (9782)$$

$$\tau^3_{\gamma,\delta,w} = \sum_{\epsilon \in A} Z^*_{\epsilon,\delta} \tau^1_{\gamma,\epsilon,w} \tau^2_{\gamma,\epsilon,w} \quad (3r_D r_T^3) \quad (9795)$$

$$\tau^4_{\gamma,i,j} = \sum_{\alpha \in B} W^1_{j,\alpha} \tau^0_{\gamma,\alpha} \tau^3_{\gamma,\alpha,i} \quad (3r_T r_V N_o^2) \quad (9783)$$

$$\tau^4_{\gamma,\delta,w} = \sum_{\epsilon \in A} Z_{\epsilon,\gamma} \tau^3_{\epsilon,\delta,w} \quad (2r_D r_T^3) \quad (9796)$$

$$\tau^5_{\gamma,i,j} = \sum_{\delta \in A} Z_{\delta,\gamma} \tau^4_{\delta,i,j} \quad (2r_T^2 N_o^2) \quad (9784)$$

$$\tau^5_{\alpha,i} = \sum_{a \in V} {}^1T_{a,i} W^2_{a,\alpha} \quad (2r_V N_o N_v) \quad (9797)$$

$$\tau^6_{\gamma,\delta,w} = \sum_{a \in V} {}^2D^1_{a,w} Y^3_{a,\gamma} Y^{1,*}_{a,\delta} \quad (3r_D r_T^2 N_v) \quad (9785)$$

$$\tau^6_{\alpha,\beta} = \sum_{i \in O} W^3_{i,\beta} \tau^5_{\alpha,i} \quad (2r_V^2 N_o) \quad (9798)$$

$$\tau^7_{\gamma,\delta,w} = \sum_{i \in O} {}^2D^2_{i,w} Y^4_{i,\gamma} Y^{2,*}_{i,\delta} \quad (3r_D r_T^2 N_o) \quad (9786)$$

$$\tau^7_{\alpha,i} = \sum_{\beta \in B} W^1_{i,\beta} X_{\beta,\alpha} \tau^6_{\beta,\alpha} \quad (3r_V^2 N_o) \quad (9799)$$

$$\tau^8_{\gamma,\delta,w} = \sum_{\epsilon \in A} Z^*_{\epsilon,\delta} \tau^6_{\gamma,\epsilon,w} \tau^7_{\gamma,\epsilon,w} \quad (3r_D r_T^3) \quad (9787)$$

$$\tau^8_{i,a} = \sum_{\alpha \in B} W^4_{a,\alpha} \tau^7_{\alpha,i} \quad (2r_V N_o N_v) \quad (9800)$$

$$\tau^9_{\gamma,w,i,j} = \sum_{\delta \in A} \tau^5_{\delta,i,j} \tau^8_{\delta,\gamma,w} \quad (2r_D r_T^2 N_o^2) \quad (9788)$$

$$\tau^9_{\gamma,i} = \sum_{a \in V} Y^3_{a,\gamma} \tau^8_{i,a} \quad (2r_T N_o N_v) \quad (9801)$$

$$\tau^{10}_{\gamma,w,i} = \sum_{j \in O} {}^2D^4_{j,w} Y^{4,*}_{j,\gamma} \tau^9_{\gamma,w,j,i} \quad (3r_D r_T N_o^2) \quad (9789)$$

$$\tau^{10}_{\gamma,w,i} = \sum_{\delta \in A} \tau^9_{\delta,i} \tau^0_{\delta,\gamma,w} \tau^4_{\delta,\gamma,w} \quad (3r_D r_T^2 N_o) \quad (9802)$$

$${}^2R^3_{a,\gamma} \leftarrow \sum_{w \in D} \sum_{i \in O} \frac{1}{2} {}^2D^3_{a,w} {}^1T_{a,i} \tau^{10}_{\gamma,w,i} \quad (3r_D r_T N_o N_v) \quad (9790)$$

$${}^2R^3_{a,\gamma} \leftarrow \sum_{w \in D} \sum_{i \in O} \frac{1}{2} {}^2D^3_{a,w} {}^1T_{a,i} \tau^{10}_{\gamma,w,i} \quad (3r_D r_T N_o N_v) \quad (9803)$$

Raw expression

$${}^2R^3_{b,\zeta} \leftarrow - \sum_{\gamma \in A} \sum_{i \in O} \sum_{j \in O} \sum_{k \in O} \sum_{l \in O} \sum_{a \in V} \sum_{c \in V} \sum_{d \in V} {}^1T_{b,k} \\ {}^1T_{c,j} Y^{1,*}_{a,\gamma} Y^{2,*}_{i,\gamma} Z^*_{\gamma,\zeta} \\ Y^{4,*}_{j,\zeta} {}^2D^{a,i,b,j} {}^2T_{a,i,d,l} V_{k,c,l,d} \quad (9791)$$

Factorized expression

$$\tau^0_{\gamma,\delta,w} = \sum_{i \in O} {}^2D^4_{i,w} Y^4_{i,\gamma} Y^{4,*}_{i,\delta} \quad (3r_D r_T^2 N_o) \quad (9792)$$

Raw expression

$${}^2R^3_{b,\zeta} \leftarrow - \sum_{\gamma \in A} \sum_{i \in O} \sum_{j \in O} \sum_{k \in O} \sum_{l \in O} \sum_{a \in V} \sum_{c \in V} \sum_{d \in V} {}^1T_{b,k} \\ {}^1T_{c,j} Y^{1,*}_{a,\gamma} Y^{2,*}_{i,\gamma} Z^*_{\gamma,\zeta} \\ Y^{4,*}_{j,\zeta} {}^2D^{a,i,b,j} {}^2T_{d,l,a,i} V_{k,c,l,d} \quad (9804)$$

Factorized expression

$$\tau^0_{\gamma,\delta,w} = \sum_{i \in O} {}^2D^4_{i,w} Y^2_{i,\gamma} Y^{4,*}_{i,\delta} \quad (3r_D r_T^2 N_o) \quad (9805)$$

$$\tau^1_{\gamma,\delta,w} = \sum_{a \in V} {}^2D^1_{a,w} Y^3_{a,\gamma} Y^{1,*}_{a,\delta} \quad (3r_D r_T^2 N_v) \quad (9806)$$

$$\tau^2_{\gamma,\delta,w} = \sum_{i \in O} {}^2D^2_{i,w} Y^4_{i,\gamma} Y^{2,*}_{i,\delta} \quad (3r_D r_T^2 N_o) \quad (9807)$$

$$\tau^3_{\gamma,\delta,w} = \sum_{\epsilon \in A} Z^*_{\epsilon,\delta} \tau^1_{\gamma,\epsilon,w} \tau^2_{\gamma,\epsilon,w} \quad (3r_D r_T^3) \quad (9808)$$

$$\tau^4_{\gamma,\delta,w} = \sum_{\epsilon \in A} Z_{\gamma,\epsilon} \tau^3_{\epsilon,\delta,w} \quad (2r_D r_T^3) \quad (9809)$$

$$\tau^5_{\alpha,i} = \sum_{a \in V} {}^1T_{a,i} W^2_{a,\alpha} \quad (2r_V N_o N_v) \quad (9810)$$

$$\tau^6_{\alpha,\beta} = \sum_{i \in O} W^3_{i,\beta} \tau^5_{\alpha,i} \quad (2r_V^2 N_o) \quad (9811)$$

$$\tau^7_{\alpha,i} = \sum_{\beta \in B} W^1_{i,\beta} X_{\beta,\alpha} \tau^6_{\beta,\alpha} \quad (3r_V^2 N_o) \quad (9812)$$

$$\tau^8_{i,a} = \sum_{\alpha \in B} W^4_{a,\alpha} \tau^7_{\alpha,i} \quad (2r_V N_o N_v) \quad (9813)$$

$$\tau^9_{\gamma,i} = \sum_{a \in V} Y^1_{a,\gamma} \tau^8_{i,a} \quad (2r_T N_o N_v) \quad (9814)$$

$$\tau^{10}_{\gamma,w,i} = \sum_{\delta \in A} \tau^9_{\delta,i} \tau^0_{\delta,\gamma,w} \tau^4_{\delta,\gamma,w} \quad (3r_D r_T^2 N_o) \quad (9815)$$

$${}^2R^3_{a,\gamma} \leftarrow \sum_{w \in D} \sum_{i \in O} \frac{1}{2} {}^2D^3_{a,w} {}^1T_{a,i} \tau^{10}_{\gamma,w,i} \quad (3r_D r_T N_o N_v) \quad (9816)$$

Raw expression

$${}^2R^3_{b,\zeta} \leftarrow - \sum_{\gamma \in A} \sum_{i \in O} \sum_{j \in O} \sum_{k \in O} \sum_{l \in O} \sum_{a \in V} \sum_{c \in V} \sum_{d \in V} {}^1T_{b,k} \\ {}^1T_{c,l} Y^{1,*}_{a,\gamma} Y^{2,*}_{i,\gamma} Z^*_{\gamma,\zeta} \\ Y^{4,*}_{j,\zeta} {}^2D^{a,i,b,j} {}^2T_{a,i,d,j} V_{k,d,l,c} \quad (9817)$$

Factorized expression

$$\tau^0_{\alpha,i} = \sum_{a \in V} {}^1T_{a,i} W^2_{a,\alpha} \quad (2r_V N_o N_v) \quad (9818)$$

$$\tau^1_{\gamma,\alpha,w} = \sum_{i \in O} {}^2D^2_{i,w} Y^{2,*}_{i,\gamma} \tau^0_{\alpha,i} \quad (3r_D r_T r_V N_o) \quad (9819)$$

$$\tau^2_{\gamma,\delta,w} = \sum_{a \in V} {}^2D^1_{a,w} Y^1_{a,\gamma} Y^{1,*}_{a,\delta} \quad (3r_D r_T^2 N_v) \quad (9820)$$

$$\tau^3_{\gamma,\delta,w,i} = \sum_{\epsilon \in A} Y^2_{i,\epsilon} Z_{\epsilon,\gamma} \tau^2_{\epsilon,\delta,w} \quad (3r_D r_T^3 N_o) \quad (9821)$$

$$\tau^4_{\gamma,\delta,\alpha,w} = \sum_{i \in O} W^1_{i,\alpha} \tau^1_{\delta,\alpha,w} \tau^3_{\gamma,\delta,w,i} \quad (3r_D r_T^2 r_V N_o) \quad (9822)$$

$$\tau^5_{\alpha,i} = \sum_{a \in V} {}^1T_{a,i} W^4_{a,\alpha} \quad (2r_V N_o N_v) \quad (9823)$$

$$\tau^6_{\alpha,i,j} = \sum_{\beta \in B} X_{\alpha,\beta} W^3_{j,\beta} \tau^5_{\beta,i} \quad (3r_V^2 N_o^2) \quad (9824)$$

$$\tau^7_{\gamma,\alpha,i} = \sum_{j \in O} Y^4_{j,\gamma} \tau^6_{\alpha,i,j} \quad (2r_T r_V N_o^2) \quad (9825)$$

$$\tau^8_{\gamma,\delta,w,i} = \sum_{\alpha \in B} \tau^7_{\gamma,\alpha,i} \tau^4_{\gamma,\delta,\alpha,w} \quad (2r_D r_T^2 r_V N_o) \quad (9826)$$

$$\tau^9_{\gamma,\delta,w} = \sum_{\epsilon \in A} \sum_{i \in O} {}^2D^4_{i,w} Z^*_{\epsilon,\delta} Y^{4,*}_{i,\delta} \tau^8_{\gamma,\epsilon,w,i} \quad (4r_D r_T^3 N_o) \quad (9827)$$

$${}^2R^3_{a,\gamma} \leftarrow \sum_{\delta \in A} \sum_{w \in D} \frac{1}{2} {}^2D^3_{a,w} Y^3_{a,\delta} \tau^9_{\delta,\gamma,w} \quad (3r_D r_T^2 N_v) \quad (9828)$$

Raw expression

$${}^2R^3_{b,\zeta} \leftarrow - \sum_{\gamma \in A} \sum_{i \in O} \sum_{j \in O} \sum_{k \in O} \sum_{l \in O} \sum_{a \in V} \sum_{c \in V} \sum_{d \in V} {}^1T_{b,k} \\ {}^1T_{c,l} Y^{1,*}_{a,\gamma} Y^{2,*}_{i,\gamma} Z^*_{\gamma,\zeta} \\ Y^{4,*}_{j,\zeta} {}^2D^{a,i,b,j} {}^2T_{d,j,a,i} V_{k,d,l,c} \quad (9829)$$

Factorized expression

$$\tau^0_{\gamma,\delta,w} = \sum_{i \in O} {}^2D^4_{i,w} Y^4_{i,\gamma} Y^{4,*}_{i,\delta} \quad (3r_D r_T^2 N_o) \quad (9830)$$

$$\tau^1_{\gamma,\delta,w} = \sum_{a \in V} {}^2D^1_{a,w} Y^1_{a,\gamma} Y^{1,*}_{a,\delta} \quad (3r_D r_T^2 N_v) \quad (9831)$$

$$\tau^1_{\gamma,\delta,w} = \sum_{a \in V} {}^2D^1_{a,w} Y^3_{a,\gamma} Y^{1,*}_{a,\delta} \quad (3r_D r_T^2 N_v) \quad (9844)$$

$$\tau^2_{\alpha,i} = \sum_{a \in V} {}^1T_{a,i} W^4_{a,\alpha} \quad (2r_V N_o N_v) \quad (9832)$$

$$\tau^2_{\alpha,i} = \sum_{a \in V} {}^1T_{a,i} W^4_{a,\alpha} \quad (2r_V N_o N_v) \quad (9845)$$

$$\tau^3_{\alpha,\beta} = \sum_{i \in O} W^1_{i,\alpha} \tau^2_{\beta,i} \quad (2r_V^2 N_o) \quad (9833)$$

$$\tau^3_{\alpha,\beta} = \sum_{i \in O} W^1_{i,\alpha} \tau^2_{\beta,i} \quad (2r_V^2 N_o) \quad (9846)$$

$$\tau^4_{\alpha,i} = \sum_{\beta \in B} X_{\alpha,\beta} W^3_{i,\beta} \tau^3_{\alpha,\beta} \quad (3r_V^2 N_o) \quad (9834)$$

$$\tau^4_{\alpha,i} = \sum_{\beta \in B} X_{\alpha,\beta} W^3_{i,\beta} \tau^3_{\alpha,\beta} \quad (3r_V^2 N_o) \quad (9847)$$

$$\tau^5_{\alpha,i} = \sum_{\alpha \in B} W^2_{a,\alpha} \tau^4_{\alpha,i} \quad (2r_V N_o N_v) \quad (9835)$$

$$\tau^5_{i,a} = \sum_{\alpha \in B} W^2_{a,\alpha} \tau^4_{\alpha,i} \quad (2r_V N_o N_v) \quad (9848)$$

$$\tau^6_{i,j} = \sum_{a \in V} {}^1T_{a,i} \tau^5_{j,a} \quad (2N_o^2 N_v) \quad (9836)$$

$$\tau^6_{i,j} = \sum_{a \in V} {}^1T_{a,i} \tau^5_{j,a} \quad (2N_o^2 N_v) \quad (9849)$$

$$\tau^7_{\gamma,i} = \sum_{j \in O} Y^2_{j,\gamma} \tau^6_{i,j} \quad (2r_T N_o^2) \quad (9837)$$

$$\tau^7_{\gamma,i} = \sum_{j \in O} Y^4_{j,\gamma} \tau^6_{i,j} \quad (2r_T N_o^2) \quad (9850)$$

$$\tau^8_{\gamma,\delta,w} = \sum_{i \in O} {}^2D^2_{i,w} Y^{2,*}_{i,\delta} \tau^7_{\gamma,i} \quad (3r_D r_T^2 N_o) \quad (9838)$$

$$\tau^8_{\gamma,\delta,w} = \sum_{i \in O} {}^2D^2_{i,w} Y^{2,*}_{i,\delta} \tau^7_{\gamma,i} \quad (3r_D r_T^2 N_o) \quad (9851)$$

$$\tau^9_{\gamma,\delta,w} = \sum_{\epsilon \in A} Z^*_{\epsilon,\delta} \tau^1_{\gamma,\epsilon,w} \tau^8_{\gamma,\epsilon,w} \quad (3r_D r_T^3) \quad (9839)$$

$$\tau^9_{\gamma,\delta,w} = \sum_{\epsilon \in A} Z^*_{\epsilon,\delta} \tau^1_{\gamma,\epsilon,w} \tau^8_{\gamma,\epsilon,w} \quad (3r_D r_T^3) \quad (9852)$$

$$\tau^{10}_{\gamma,\delta,w} = \sum_{\epsilon \in A} Z_{\epsilon,\gamma} \tau^9_{\epsilon,\delta,w} \quad (2r_D r_T^3) \quad (9840)$$

$$\tau^{10}_{\gamma,\delta,w} = \sum_{\epsilon \in A} Z_{\gamma,\epsilon} \tau^9_{\epsilon,\delta,w} \quad (2r_D r_T^3) \quad (9853)$$

$${}^2R^3_{a,\gamma} \leftarrow \sum_{\delta \in A} \sum_{w \in D} \frac{1}{2} {}^2D^3_{a,w} Y^3_{a,\delta} \tau^0_{\delta,\gamma,w} \tau^{10}_{\delta,\gamma,w} \quad (4r_D r_T^2 N_v) \quad (9841)$$

$${}^2R^3_{a,\gamma} \leftarrow \sum_{\delta \in A} \sum_{w \in D} \frac{1}{2} {}^2D^3_{a,w} Y^1_{a,\delta} \tau^0_{\delta,\gamma,w} \tau^{10}_{\delta,\gamma,w} \quad (4r_D r_T^2 N_v) \quad (9854)$$

Raw expression

$${}^2R^3_{b,\zeta} \leftarrow - \sum_{\gamma \in A} \sum_{i \in O} \sum_{j \in O} \sum_{k \in O} \sum_{l \in O} \sum_{a \in V} \sum_{c \in V} \sum_{d \in V} {}^1T_{c,i} \\ {}^1T_{d,k} Y^{1,*}_{a,\gamma} Y^{2,*}_{i,\gamma} Z^*_{\gamma,\zeta} \\ Y^{4,*}_{j,\zeta} {}^2D^{a,i,b,j} {}^2T_{a,l,b,j} V_{k,d,l,c} \quad (9842)$$

Raw expression

$${}^2R^3_{b,\zeta} \leftarrow - \sum_{\gamma \in A} \sum_{i \in O} \sum_{j \in O} \sum_{k \in O} \sum_{l \in O} \sum_{a \in V} \sum_{c \in V} \sum_{d \in V} {}^1T_{c,i} \\ {}^1T_{d,k} Y^{1,*}_{a,\gamma} Y^{2,*}_{i,\gamma} Z^*_{\gamma,\zeta} \\ Y^{4,*}_{j,\zeta} {}^2D^{a,i,b,j} {}^2T_{b,j,a,l} V_{k,d,l,c} \quad (9855)$$

Factorized expression

$$\tau^0_{\gamma,\delta,w} = \sum_{i \in O} {}^2D^4_{i,w} Y^2_{i,\gamma} Y^{4,*}_{i,\delta} \quad (3r_D r_T^2 N_o) \quad (9843)$$

Factorized expression

$$\tau^0_{\alpha,i} = \sum_{a \in V} {}^1T_{a,i} W^4_{a,\alpha} \quad (2r_V N_o N_v) \quad (9856)$$

$$\tau^1_{\gamma,\alpha,w} = \sum_{i \in O} {}^2D^2_{i,w} Y^{2,*}_{i,\gamma} \tau^0_{\alpha,i} \quad (3r_D r_T r_V N_o) \quad (9857)$$

$$\tau^2_{\gamma,\delta,w} = \sum_{a \in V} {}^2D^1_{a,w} Y^3_{a,\gamma} Y^{1,*}_{a,\delta} \quad (3r_D r_T^2 N_v) \quad (9858)$$

$$\tau^3_{\gamma,\delta,w,i} = \sum_{\epsilon \in A} Z_{\gamma,\epsilon} Y^4_{i,\epsilon} \tau^2_{\epsilon,\delta,w} \quad (3r_D r_T^3 N_o) \quad (9859)$$

$$\tau^4_{\gamma,\delta,\alpha,w} = \sum_{i \in O} W^3_{i,\alpha} \tau^1_{\delta,\alpha,w} \tau^3_{\gamma,\delta,w,i} \quad (3r_D r_T^2 r_V N_o) \quad (9860)$$

$$\tau^5_{\alpha,i} = \sum_{a \in V} {}^1T_{a,i} W^2_{a,\alpha} \quad (2r_V N_o N_v) \quad (9861)$$

$$\tau^6_{\alpha,i,j} = \sum_{\beta \in B} W^1_{j,\beta} X_{\beta,\alpha} \tau^5_{\beta,i} \quad (3r_V^2 N_o^2) \quad (9862)$$

$$\tau^7_{\gamma,\alpha,i} = \sum_{j \in O} Y^2_{j,\gamma} \tau^6_{\alpha,i,j} \quad (2r_T r_V N_o^2) \quad (9863)$$

$$\tau^8_{\gamma,\delta,w,i} = \sum_{\alpha \in B} \tau^7_{\gamma,\alpha,i} \tau^4_{\gamma,\delta,\alpha,w} \quad (2r_D r_T^2 r_V N_o) \quad (9864)$$

$$\tau^9_{\gamma,\delta,w} = \sum_{\epsilon \in A} \sum_{i \in O} {}^2D^4_{i,w} Z^*_{\epsilon,\delta} Y^{4,*}_{i,\delta} \tau^8_{\gamma,\epsilon,w,i} \quad (4r_D r_T^3 N_o) \quad (9865)$$

$${}^2R^3_{a,\gamma} \leftarrow \sum_{\delta \in A} \sum_{w \in D} \frac{1}{2} {}^2D^3_{a,w} Y^1_{a,\delta} \tau^9_{\delta,\gamma,w} \quad (3r_D r_T^2 N_v) \quad (9866)$$

Raw expression

$${}^2R^3_{b,\zeta} \leftarrow - \sum_{\gamma \in A} \sum_{i \in O} \sum_{j \in O} \sum_{k \in O} \sum_{l \in O} \sum_{a \in V} \sum_{c \in V} \sum_{d \in V} {}^1T_{c,j} \\ {}^1T_{d,k} Y^{1,*}_{a,\gamma} Y^{2,*}_{i,\gamma} Z^*_{\gamma,\zeta} \\ Y^{4,*}_{j,\zeta} {}^2D^{a,i,b,j} {}^2T_{a,i,b,l} V_{k,d,l,c} \quad (9867)$$

Factorized expression

$$\tau^0_{\alpha,i} = \sum_{a \in V} {}^1T_{a,i} W^4_{a,\alpha} \quad (2r_V N_o N_v) \quad (9868)$$

$$\tau^1_{\alpha,\beta} = \sum_{i \in O} W^1_{i,\alpha} \tau^0_{\beta,i} \quad (2r_V^2 N_o) \quad (9869)$$

$$\tau^2_{\alpha,i} = \sum_{\beta \in B} X_{\alpha,\beta} W^3_{i,\beta} \tau^1_{\alpha,\beta} \quad (3r_V^2 N_o) \quad (9870)$$

$$\tau^3_{i,a} = \sum_{\alpha \in B} W^2_{a,\alpha} \tau^2_{\alpha,i} \quad (2r_V N_o N_v) \quad (9871)$$

$$\tau^4_{i,j} = \sum_{a \in V} {}^1T_{a,i} \tau^3_{j,a} \quad (2N_o^2 N_v) \quad (9872)$$

$$\tau^5_{\gamma,i} = \sum_{j \in O} Y^4_{j,\gamma} \tau^4_{i,j} \quad (2r_T N_o^2) \quad (9873)$$

$$\tau^6_{\gamma,\delta,w} = \sum_{i \in O} {}^2D^4_{i,w} Y^{4,*}_{i,\delta} \tau^5_{\gamma,i} \quad (3r_D r_T^2 N_o) \quad (9874)$$

$$\tau^7_{\gamma,\delta,w} = \sum_{a \in V} {}^2D^1_{a,w} Y^1_{a,\gamma} Y^{1,*}_{a,\delta} \quad (3r_D r_T^2 N_v) \quad (9875)$$

$$\tau^8_{\gamma,\delta,w} = \sum_{i \in O} {}^2D^2_{i,w} Y^2_{i,\gamma} Y^{2,*}_{i,\delta} \quad (3r_D r_T^2 N_o) \quad (9876)$$

$$\tau^9_{\gamma,\delta,w} = \sum_{\epsilon \in A} Z^*_{\epsilon,\delta} \tau^7_{\gamma,\epsilon,w} \tau^8_{\gamma,\epsilon,w} \quad (3r_D r_T^3) \quad (9877)$$

$$\tau^{10}_{\gamma,\delta,w} = \sum_{\epsilon \in A} Z_{\epsilon,\gamma} \tau^9_{\epsilon,\delta,w} \quad (2r_D r_T^3) \quad (9878)$$

$${}^2R^3_{a,\gamma} \leftarrow \sum_{\delta \in A} \sum_{w \in D} \frac{1}{2} {}^2D^3_{a,w} Y^3_{a,\delta} \tau^{10}_{\delta,\gamma,w} \tau^6_{\delta,\gamma,w} \quad (4r_D r_T^2 N_v) \quad (9879)$$

Raw expression

$${}^2R^3_{b,\zeta} \leftarrow - \sum_{\gamma \in A} \sum_{i \in O} \sum_{j \in O} \sum_{k \in O} \sum_{l \in O} \sum_{a \in V} \sum_{c \in V} \sum_{d \in V} {}^1T_{c,j} \\ {}^1T_{d,k} Y^{1,*}_{a,\gamma} Y^{2,*}_{i,\gamma} Z^*_{\gamma,\zeta} \\ Y^{4,*}_{j,\zeta} {}^2D^{a,i,b,j} {}^2T_{b,l,a,i} V_{k,d,l,c} \quad (9880)$$

Factorized expression

$$\tau^0_{\alpha,i} = \sum_{a \in V} {}^1T_{a,i} W^4_{a,\alpha} \quad (2r_V N_o N_v) \quad (9881)$$

$$\tau^1_{\alpha,\beta} = \sum_{i \in O} W^1_{i,\alpha} \tau^0_{\beta,i} \quad (2r_V^2 N_o) \quad (9882)$$

$$\tau^0_{\gamma,\delta,w} = \sum_{a \in V} {}^2D^1_{a,w} Y^1_{a,\gamma} Y^{1,*}_{a,\delta} \quad (3r_D r_T^2 N_v) \quad (9894)$$

$$\tau^2_{\alpha,i} = \sum_{\beta \in B} X_{\alpha,\beta} W^3_{i,\beta} \tau^1_{\alpha,\beta} \quad (3r_V^2 N_o) \quad (9883)$$

$$\tau^1_{\gamma,\delta,w} = \sum_{i \in O} {}^2D^2_{i,w} Y^2_{i,\gamma} Y^{2,*}_{i,\delta} \quad (3r_D r_T^2 N_o) \quad (9895)$$

$$\tau^3_{i,a} = \sum_{\alpha \in B} W^2_{a,\alpha} \tau^2_{\alpha,i} \quad (2r_V N_o N_v) \quad (9884)$$

$$\tau^2_{\gamma,\delta,w} = \sum_{\epsilon \in A} Z^*_{\epsilon,\delta} \tau^0_{\gamma,\epsilon,w} \tau^1_{\gamma,\epsilon,w} \quad (3r_D r_T^3) \quad (9896)$$

$$\tau^4_{i,j} = \sum_{a \in V} {}^1T_{a,i} \tau^3_{j,a} \quad (2N_o^2 N_v) \quad (9885)$$

$$\tau^3_{\gamma,\alpha} = \sum_{a \in V} W^4_{a,\alpha} Y^3_{a,\gamma} \quad (2r_T r_V N_v) \quad (9897)$$

$$\tau^5_{\gamma,i} = \sum_{j \in O} Y^2_{j,\gamma} \tau^4_{i,j} \quad (2r_T N_o^2) \quad (9886)$$

$$\tau^4_{\gamma,\alpha} = \sum_{i \in O} W^3_{i,\alpha} Y^4_{i,\gamma} \quad (2r_T r_V N_o) \quad (9898)$$

$$\tau^6_{\gamma,\delta,w} = \sum_{i \in O} {}^2D^4_{i,w} Y^{4,*}_{i,\delta} \tau^5_{\gamma,i} \quad (3r_D r_T^2 N_o) \quad (9887)$$

$$\tau^5_{\gamma,\alpha} = \sum_{\beta \in B} X_{\alpha,\beta} \tau^3_{\gamma,\beta} \tau^4_{\gamma,\beta} \quad (3r_T r_V^2) \quad (9899)$$

$$\tau^7_{\gamma,\delta,w} = \sum_{a \in V} {}^2D^1_{a,w} Y^3_{a,\gamma} Y^{1,*}_{a,\delta} \quad (3r_D r_T^2 N_v) \quad (9888)$$

$$\tau^6_{\gamma,\alpha} = \sum_{a \in V} W^2_{a,\alpha} Y^3_{a,\gamma} \quad (2r_T r_V N_v) \quad (9900)$$

$$\tau^8_{\gamma,\delta,w} = \sum_{i \in O} {}^2D^2_{i,w} Y^4_{i,\gamma} Y^{2,*}_{i,\delta} \quad (3r_D r_T^2 N_o) \quad (9889)$$

$$\tau^7_{\gamma,\alpha} = \sum_{i \in O} W^1_{i,\alpha} Y^4_{i,\gamma} \quad (2r_T r_V N_o) \quad (9901)$$

$$\tau^9_{\gamma,\delta,w} = \sum_{\epsilon \in A} Z^*_{\epsilon,\delta} \tau^7_{\gamma,\epsilon,w} \tau^8_{\gamma,\epsilon,w} \quad (3r_D r_T^3) \quad (9890)$$

$$\tau^8_{\gamma,\delta} = \sum_{\alpha \in B} \tau^5_{\delta,\alpha} \tau^6_{\gamma,\alpha} \tau^7_{\gamma,\alpha} \quad (3r_T^2 r_V) \quad (9902)$$

$$\tau^{10}_{\gamma,\delta,w} = \sum_{\epsilon \in A} Z_{\gamma,\epsilon} \tau^9_{\epsilon,\delta,w} \quad (2r_D r_T^3) \quad (9891)$$

$$\tau^9_{\gamma,\delta} = \sum_{\epsilon \in A} Z_{\gamma,\epsilon} \tau^8_{\delta,\epsilon} \quad (2r_T^3) \quad (9903)$$

$${}^2R^3_{a,\gamma} \leftarrow \sum_{\delta \in A} \sum_{w \in D} \frac{1}{2} {}^2D^3_{a,w} Y^1_{a,\delta} \tau^{10}_{\delta,\gamma,w} \tau^6_{\delta,\gamma,w} \quad (4r_D r_T^2 N_v) \quad (9892)$$

$$\tau^{10}_{\gamma,\delta} = \sum_{\epsilon \in A} Z_{\gamma,\epsilon} \tau^9_{\delta,\epsilon} \quad (2r_T^3) \quad (9904)$$

$$\tau^{11}_{\gamma,\delta,w} = \sum_{\epsilon \in A} \tau^{10}_{\epsilon,\gamma} \tau^2_{\epsilon,\delta,w} \quad (2r_D r_T^3) \quad (9905)$$

### I. Contributions from $(H^2 T^2 T)_c$

Raw expression

$${}^2R^3_{b,\zeta} \leftarrow \sum_{\gamma \in A} \sum_{i \in O} \sum_{j \in O} \sum_{k \in O} \sum_{l \in O} \sum_{a \in V} \sum_{c \in V} \sum_{d \in V} Y^{1,*}_{a,\gamma} Y^{2,*}_{i,\gamma} Z^*_{\gamma,\zeta} Y^{4,*}_{j,\zeta} {}^2D^{a,i,b,j} {}^2T_{a,i,d,l} {}^2T_{b,j,c,k} V_{l,d,k,c} \quad (9893)$$

Factorized expression

$$\tau^{12}_{\gamma,\delta,w} = \sum_{i \in O} {}^2D^4_{i,w} Y^2_{i,\gamma} Y^{4,*}_{i,\delta} \quad (3r_D r_T^2 N_o) \quad (9906)$$

$${}^2R^3_{a,\gamma} \leftarrow \sum_{\delta \in A} \sum_{w \in D} {}^2D^3_{a,w} Y^1_{a,\delta} \tau^{11}_{\delta,\gamma,w} \tau^{12}_{\delta,\gamma,w} \quad (4r_D r_T^2 N_v) \quad (9907)$$

Raw expression

$${}^2R^3_{b,\zeta} \leftarrow \sum_{\gamma \in A} \sum_{i \in O} \sum_{j \in O} \sum_{k \in O} \sum_{l \in O} \sum_{a \in V} \sum_{c \in V} \sum_{d \in V} Y^{1,*}_{a,\gamma} Y^{2,*}_{i,\gamma} Z^*_{\gamma,\zeta} Y^{4,*}_{j,\zeta} {}^2D^{a,i,b,j} {}^2T_{a,i,d,l} {}^2T_{c,k,b,j} V_{l,d,k,c} \quad (9908)$$

Factorized expression

$$\tau^0_{\gamma,\delta,w} = \sum_{a \in V} {}^2D^1_{a,w} Y^1_{a,\gamma} Y^{1,*}_{a,\delta} \quad (3r_D r_T^2 N_v) \quad (9909)$$

$$\tau^1_{\gamma,\delta,w} = \sum_{i \in O} {}^2D^2_{i,w} Y^2_{i,\gamma} Y^{2,*}_{i,\delta} \quad (3r_D r_T^2 N_o) \quad (9910)$$

$$\tau^2_{\gamma,\delta,w} = \sum_{\epsilon \in A} Z^*_{\epsilon,\delta} \tau^0_{\gamma,\epsilon,w} \tau^1_{\gamma,\epsilon,w} \quad (3r_D r_T^3) \quad (9911)$$

$$\tau^3_{\gamma,\alpha} = \sum_{a \in V} W^2_{a,\alpha} Y^3_{a,\gamma} \quad (2r_T r_V N_v) \quad (9912)$$

$$\tau^4_{\gamma,\alpha} = \sum_{i \in O} W^1_{i,\alpha} Y^4_{i,\gamma} \quad (2r_T r_V N_o) \quad (9913)$$

$$\tau^5_{\gamma,\alpha} = \sum_{a \in V} W^4_{a,\alpha} Y^1_{a,\gamma} \quad (2r_T r_V N_v) \quad (9914)$$

$$\tau^6_{\gamma,\alpha} = \sum_{i \in O} W^3_{i,\alpha} Y^2_{i,\gamma} \quad (2r_T r_V N_o) \quad (9915)$$

$$\tau^7_{\gamma,\alpha} = \sum_{\beta \in B} X_{\alpha,\beta} \tau^5_{\gamma,\beta} \tau^6_{\gamma,\beta} \quad (3r_T r_V^2) \quad (9916)$$

$$\tau^8_{\gamma,\delta} = \sum_{\alpha \in B} \tau^3_{\delta,\alpha} \tau^4_{\delta,\alpha} \tau^7_{\gamma,\alpha} \quad (3r_T^2 r_V) \quad (9917)$$

$$\tau^9_{\gamma,\delta} = \sum_{\epsilon \in A} Z_{\delta,\epsilon} \tau^8_{\gamma,\epsilon} \quad (2r_T^3) \quad (9918)$$

$$\tau^{10}_{\gamma,\delta} = \sum_{\epsilon \in A} Z_{\epsilon,\delta} \tau^9_{\epsilon,\gamma} \quad (2r_T^3) \quad (9919)$$

$$\tau^{11}_{\gamma,\delta,w} = \sum_{\epsilon \in A} \tau^{10}_{\epsilon,\gamma} \tau^2_{\epsilon,\delta,w} \quad (2r_D r_T^3) \quad (9920)$$

$$\tau^{12}_{\gamma,\delta,w} = \sum_{i \in O} {}^2D^4_{i,w} Y^4_{i,\gamma} Y^{4,*}_{i,\delta} \quad (3r_D r_T^2 N_o) \quad (9921)$$

$${}^2R^3_{a,\gamma} \leftarrow \sum_{\delta \in A} \sum_{w \in D} {}^2D^3_{a,w} Y^3_{a,\delta} \tau^{11}_{\delta,\gamma,w} \tau^{12}_{\delta,\gamma,w} \quad (4r_D r_T^2 N_v) \quad (9922)$$

Raw expression

$${}^2R^3_{b,\zeta} \leftarrow \sum_{\gamma \in A} \sum_{i \in O} \sum_{j \in O} \sum_{k \in O} \sum_{l \in O} \sum_{a \in V} \sum_{c \in V} \sum_{d \in V} Y^{1,*}_{a,\gamma} Y^{2,*}_{i,\gamma} Z^*_{\gamma,\zeta} Y^{4,*}_{j,\zeta} {}^2D^{a,i,b,j} {}^2T_{b,j,c,k} {}^2T_{d,l,a,i} V_{l,d,k,c} \quad (9923)$$

Factorized expression

$$\tau^0_{\gamma,\delta,w} = \sum_{a \in V} {}^2D^1_{a,w} Y^3_{a,\gamma} Y^{1,*}_{a,\delta} \quad (3r_D r_T^2 N_v) \quad (9924)$$

$$\tau^1_{\gamma,\delta,w} = \sum_{i \in O} {}^2D^2_{i,w} Y^4_{i,\gamma} Y^{2,*}_{i,\delta} \quad (3r_D r_T^2 N_o) \quad (9925)$$

$$\tau^2_{\gamma,\delta,w} = \sum_{\epsilon \in A} Z^*_{\epsilon,\delta} \tau^0_{\gamma,\epsilon,w} \tau^1_{\gamma,\epsilon,w} \quad (3r_D r_T^3) \quad (9926)$$

$$\tau^3_{\gamma,\alpha} = \sum_{a \in V} W^4_{a,\alpha} Y^3_{a,\gamma} \quad (2r_T r_V N_v) \quad (9927)$$

$$\tau^4_{\gamma,\alpha} = \sum_{i \in O} W^3_{i,\alpha} Y^4_{i,\gamma} \quad (2r_T r_V N_o) \quad (9928)$$

$$\tau^5_{\gamma,\alpha} = \sum_{\beta \in B} X_{\alpha,\beta} \tau^3_{\gamma,\beta} \tau^4_{\gamma,\beta} \quad (3r_T r_V^2) \quad (9929)$$

$$\tau^6_{\gamma,\alpha} = \sum_{a \in V} W^2_{a,\alpha} Y^1_{a,\gamma} \quad (2r_T r_V N_v) \quad (9930)$$

$$\tau^7_{\gamma,\alpha} = \sum_{i \in O} W^1_{i,\alpha} Y^2_{i,\gamma} \quad (2r_T r_V N_o) \quad (9931)$$

$$\tau^8_{\gamma,\delta} = \sum_{\alpha \in B} \tau^5_{\delta,\alpha} \tau^6_{\gamma,\alpha} \tau^7_{\gamma,\alpha} \quad (3r_T^2 r_V) \quad (9932)$$

$$\tau^9_{\gamma,\delta} = \sum_{\epsilon \in A} Z_{\delta,\epsilon} \tau^8_{\gamma,\epsilon} \quad (2r_T^3) \quad (9933)$$

$$\tau^{10}_{\gamma,\delta} = \sum_{\epsilon \in A} Z_{\epsilon,\delta} \tau^9_{\epsilon,\gamma} \quad (2r_T^3) \quad (9934)$$

$$\tau^{11}_{\gamma,\delta,w} = \sum_{\epsilon \in A} \tau^{10}_{\gamma,\epsilon} \tau^2_{\epsilon,\delta,w} \quad (2r_D r_T^3) \quad (9935)$$

$$\tau^9_{\gamma,\delta} = \sum_{\epsilon \in A} Z_{\epsilon,\delta} \tau^8_{\gamma,\epsilon} \quad (2r_T^3) \quad (9948)$$

$$\tau^{12}_{\gamma,\delta,w} = \sum_{i \in O} {}^2D^4_{i,w} Y^2_{i,\gamma} Y^{4,*}_{i,\delta} \quad (3r_D r_T^2 N_o) \quad (9936)$$

$$\tau^{10}_{\gamma,\delta} = \sum_{\epsilon \in A} Z_{\epsilon,\gamma} \tau^9_{\epsilon,\delta} \quad (2r_T^3) \quad (9949)$$

$${}^2R^3_{a,\gamma} \leftarrow \sum_{\delta \in A} \sum_{w \in D} {}^2D^3_{a,w} Y^1_{a,\delta} \tau^{11}_{\delta,\gamma,w} \tau^{12}_{\delta,\gamma,w} \quad (4r_D r_T^2 N_v) \quad (9937)$$

$$\tau^{11}_{\gamma,\delta,w} = \sum_{\epsilon \in A} \tau^{10}_{\epsilon,\gamma} \tau^2_{\epsilon,\delta,w} \quad (2r_D r_T^3) \quad (9950)$$

Raw expression

$$\tau^{12}_{\gamma,\delta,w} = \sum_{i \in O} {}^2D^4_{i,w} Y^4_{i,\gamma} Y^{4,*}_{i,\delta} \quad (3r_D r_T^2 N_o) \quad (9951)$$

$${}^2R^3_{b,\zeta} \leftarrow \sum_{\gamma \in A} \sum_{i \in O} \sum_{j \in O} \sum_{k \in O} \sum_{l \in O} \sum_{a \in V} \sum_{c \in V} \sum_{d \in V} Y^{1,*}_{a,\gamma} Y^{2,*}_{i,\gamma} Z^*_{\gamma,\zeta} Y^{4,*}_{j,\zeta} {}^2D^{a,i,b,j} {}^2T_{c,k,b,j} {}^2T_{d,l,a,i} V_{l,d,k,c} \quad (9938)$$

$${}^2R^3_{a,\gamma} \leftarrow \sum_{\delta \in A} \sum_{w \in D} {}^2D^3_{a,w} Y^3_{a,\delta} \tau^{11}_{\delta,\gamma,w} \tau^{12}_{\delta,\gamma,w} \quad (4r_D r_T^2 N_v) \quad (9952)$$

Factorized expression

Raw expression

$$\tau^0_{\gamma,\delta,w} = \sum_{a \in V} {}^2D^1_{a,w} Y^3_{a,\gamma} Y^{1,*}_{a,\delta} \quad (3r_D r_T^2 N_v) \quad (9939)$$

$${}^2R^3_{b,\zeta} \leftarrow - \sum_{\gamma \in A} \sum_{i \in O} \sum_{j \in O} \sum_{k \in O} \sum_{l \in O} \sum_{a \in V} \sum_{c \in V} \sum_{d \in V} \frac{1}{2} Y^{1,*}_{a,\gamma} Y^{2,*}_{i,\gamma} Z^*_{\gamma,\zeta} Y^{4,*}_{j,\zeta} {}^2D^{a,i,b,j} {}^2T_{a,i,b,k} {}^2T_{c,j,d,l} V_{k,c,l,d} \quad (9953)$$

$$\tau^1_{\gamma,\delta,w} = \sum_{i \in O} {}^2D^2_{i,w} Y^4_{i,\gamma} Y^{2,*}_{i,\delta} \quad (3r_D r_T^2 N_o) \quad (9940)$$

Factorized expression

$$\tau^2_{\gamma,\delta,w} = \sum_{\epsilon \in A} Z^*_{\epsilon,\delta} \tau^0_{\gamma,\epsilon,w} \tau^1_{\gamma,\epsilon,w} \quad (3r_D r_T^3) \quad (9941)$$

$$\tau^0_{\gamma,\delta,w} = \sum_{a \in V} {}^2D^1_{a,w} Y^1_{a,\gamma} Y^{1,*}_{a,\delta} \quad (3r_D r_T^2 N_v) \quad (9954)$$

$$\tau^3_{\gamma,\alpha} = \sum_{a \in V} W^4_{a,\alpha} Y^1_{a,\gamma} \quad (2r_T r_V N_v) \quad (9942)$$

$$\tau^1_{\gamma,\delta,w} = \sum_{i \in O} {}^2D^2_{i,w} Y^2_{i,\gamma} Y^{2,*}_{i,\delta} \quad (3r_D r_T^2 N_o) \quad (9955)$$

$$\tau^4_{\gamma,\alpha} = \sum_{i \in O} W^3_{i,\alpha} Y^2_{i,\gamma} \quad (2r_T r_V N_o) \quad (9943)$$

$$\tau^2_{\gamma,\delta,w} = \sum_{\epsilon \in A} Z^*_{\epsilon,\delta} \tau^0_{\gamma,\epsilon,w} \tau^1_{\gamma,\epsilon,w} \quad (3r_D r_T^3) \quad (9956)$$

$$\tau^5_{\gamma,\alpha} = \sum_{\beta \in B} X_{\alpha,\beta} \tau^3_{\gamma,\beta} \tau^4_{\gamma,\beta} \quad (3r_T r_V^2) \quad (9944)$$

$$\tau^3_{\gamma,\delta,w} = \sum_{\epsilon \in A} Z_{\epsilon,\gamma} \tau^2_{\epsilon,\delta,w} \quad (2r_D r_T^3) \quad (9957)$$

$$\tau^6_{\gamma,\alpha} = \sum_{a \in V} W^2_{a,\alpha} Y^1_{a,\gamma} \quad (2r_T r_V N_v) \quad (9945)$$

$$\tau^4_{\gamma,\alpha} = \sum_{a \in V} W^2_{a,\alpha} Y^1_{a,\gamma} \quad (2r_T r_V N_v) \quad (9958)$$

$$\tau^7_{\gamma,\alpha} = \sum_{i \in O} W^1_{i,\alpha} Y^2_{i,\gamma} \quad (2r_T r_V N_o) \quad (9946)$$

$$\tau^5_{\gamma,\alpha} = \sum_{a \in V} W^4_{a,\alpha} Y^3_{a,\gamma} \quad (2r_T r_V N_v) \quad (9959)$$

$$\tau^8_{\gamma,\delta} = \sum_{\alpha \in B} \tau^5_{\delta,\alpha} \tau^6_{\gamma,\alpha} \tau^7_{\gamma,\alpha} \quad (3r_T^2 r_V) \quad (9947)$$

$$\tau^6_{\gamma,\alpha} = \sum_{i \in O} W^3_{i,\alpha} Y^4_{i,\gamma} \quad (2r_T r_V N_o) \quad (9960)$$

$$\tau^7_{\gamma,\alpha} = \sum_{\beta \in B} X_{\alpha,\beta} \tau^5_{\gamma,\beta} \tau^6_{\gamma,\beta} \quad (3r_T r_V^2) \quad (9961)$$

$$\tau^5_{\gamma,\alpha} = \sum_{\delta \in A} Z_{\gamma,\delta} \tau^4_{\delta,\alpha} \quad (2r_T^2 r_V) \quad (9974)$$

$$\tau^8_{\gamma,\alpha} = \sum_{\delta \in A} Z_{\gamma,\delta} \tau^7_{\delta,\alpha} \quad (2r_T^2 r_V) \quad (9962)$$

$$\tau^6_{\gamma,i} = \sum_{\alpha \in B} W^1_{i,\alpha} \tau^1_{\gamma,\alpha} \tau^5_{\gamma,\alpha} \quad (3r_T r_V N_o) \quad (9975)$$

$$\tau^9_{\gamma,i} = \sum_{\alpha \in B} W^1_{i,\alpha} \tau^4_{\gamma,\alpha} \tau^8_{\gamma,\alpha} \quad (3r_T r_V N_o) \quad (9963)$$

$$\tau^7_{i,j} = \sum_{\gamma \in A} Y^2_{j,\gamma} \tau^6_{\gamma,i} \quad (2r_T N_o^2) \quad (9976)$$

$$\tau^{10}_{i,j} = \sum_{\gamma \in A} Y^2_{j,\gamma} \tau^9_{\gamma,i} \quad (2r_T N_o^2) \quad (9964)$$

$$\tau^8_{\gamma,i} = \sum_{j \in O} Y^2_{j,\gamma} \tau^7_{j,i} \quad (2r_T N_o^2) \quad (9977)$$

$$\tau^{11}_{\gamma,i} = \sum_{j \in O} Y^4_{j,\gamma} \tau^{10}_{j,i} \quad (2r_T N_o^2) \quad (9965)$$

$$\tau^9_{\gamma,\delta,w} = \sum_{i \in O} {}^2D^2_{i,w} Y^{2,*}_{i,\delta} \tau^8_{\gamma,i} \quad (3r_D r_T^2 N_o) \quad (9978)$$

$$\tau^{12}_{\gamma,\delta,w} = \sum_{i \in O} {}^2D^4_{i,w} Y^{4,*}_{i,\delta} \tau^{11}_{\gamma,i} \quad (3r_D r_T^2 N_o) \quad (9966)$$

$$\tau^{10}_{\gamma,\delta,w} = \sum_{a \in V} {}^2D^1_{a,w} Y^1_{a,\gamma} Y^{1,*}_{a,\delta} \quad (3r_D r_T^2 N_v) \quad (9979)$$

$${}^2R^3_{a,\gamma} \leftarrow - \sum_{\delta \in A} \sum_{w \in D} \frac{1}{2} {}^2D^3_{a,w} Y^3_{a,\delta} \tau^{12}_{\delta,\gamma,w} \tau^3_{\delta,\gamma,w} \quad (4r_D r_T^2 N_v) \quad (9967)$$

$$\tau_{\gamma,\delta,w} = \sum_{\epsilon \in A} Z^*_{\epsilon,\delta} \tau^{10}_{\gamma,\epsilon,w} \tau^9_{\gamma,\epsilon,w} \quad (3r_D r_T^3) \quad (9980)$$

Raw expression

$$\tau^{12}_{\gamma,\delta,w} = \sum_{\epsilon \in A} Z_{\epsilon,\gamma} \tau^{11}_{\epsilon,\delta,w} \quad (2r_D r_T^3) \quad (9981)$$

$${}^2R^3_{b,\zeta} \leftarrow - \sum_{\gamma \in A} \sum_{i \in O} \sum_{j \in O} \sum_{k \in O} \sum_{l \in O} \sum_{a \in V} \sum_{c \in V} \sum_{d \in V} \frac{1}{2} \quad (9968)$$

$$Y^{1,*}_{a,\gamma} Y^{2,*}_{i,\gamma} Z^*_{\gamma,\zeta} Y^{4,*}_{j,\zeta} {}^2D^{a,i,b,j}_{a,i,b,j} {}^2T_{a,i,b,k} {}^2T_{c,l,d,j} V_{k,d,l,c}$$

$${}^2R^3_{a,\gamma} \leftarrow - \sum_{\delta \in A} \sum_{w \in D} \frac{1}{2} {}^2D^3_{a,w} Y^3_{a,\delta} \tau^0_{\delta,\gamma,w} \tau^{12}_{\delta,\gamma,w} \quad (4r_D r_T^2 N_v) \quad (9982)$$

Factorized expression

Raw expression

$$\tau^0_{\gamma,\delta,w} = \sum_{i \in O} {}^2D^4_{i,w} Y^4_{i,\gamma} Y^{4,*}_{i,\delta} \quad (3r_D r_T^2 N_o) \quad (9969)$$

$${}^2R^3_{b,\zeta} \leftarrow - \sum_{\gamma \in A} \sum_{i \in O} \sum_{j \in O} \sum_{k \in O} \sum_{l \in O} \sum_{a \in V} \sum_{c \in V} \sum_{d \in V} \frac{1}{2} \quad (9983)$$

$$Y^{1,*}_{a,\gamma} Y^{2,*}_{i,\gamma} Z^*_{\gamma,\zeta} Y^{4,*}_{j,\zeta} {}^2D^{a,i,b,j}_{a,i,b,j} {}^2T_{a,i,d,j} {}^2T_{b,k,c,l} V_{k,d,l,c}$$

$$\tau^1_{\gamma,\alpha} = \sum_{a \in V} W^2_{a,\alpha} Y^1_{a,\gamma} \quad (2r_T r_V N_v) \quad (9970)$$

Factorized expression

$$\tau^2_{\gamma,\alpha} = \sum_{a \in V} W^4_{a,\alpha} Y^3_{a,\gamma} \quad (2r_T r_V N_v) \quad (9971)$$

$$\tau^0_{\gamma,\delta,w} = \sum_{a \in V} {}^2D^1_{a,w} Y^1_{a,\gamma} Y^{1,*}_{a,\delta} \quad (3r_D r_T^2 N_v) \quad (9984)$$

$$\tau^3_{\gamma,\alpha} = \sum_{i \in O} W^3_{i,\alpha} Y^4_{i,\gamma} \quad (2r_T r_V N_o) \quad (9972)$$

$$\tau^1_{\gamma,\delta,w} = \sum_{i \in O} {}^2D^2_{i,w} Y^2_{i,\gamma} Y^{2,*}_{i,\delta} \quad (3r_D r_T^2 N_o) \quad (9985)$$

$$\tau^4_{\gamma,\alpha} = \sum_{\beta \in B} X_{\alpha,\beta} \tau^2_{\gamma,\beta} \tau^3_{\gamma,\beta} \quad (3r_T r_V^2) \quad (9973)$$

$$\tau^2_{\gamma,\delta,w} = \sum_{\epsilon \in A} Z^*_{\epsilon,\delta} \tau^0_{\gamma,\epsilon,w} \tau^1_{\gamma,\epsilon,w} \quad (3r_D r_T^3) \quad (9986)$$



$$\tau^3_{\gamma,\delta,w} = \sum_{\epsilon \in A} Z_{\epsilon,\gamma} \tau^2_{\epsilon,\delta,w} \quad (2r_D r_T^3) \quad (9987)$$

$$\tau^1_{\gamma,\alpha} = \sum_{a \in V} W^4_{a,\alpha} Y^1_{a,\gamma} \quad (2r_T r_V N_v) \quad (10000)$$

$$\tau^4_{\gamma,\alpha} = \sum_{a \in V} W^4_{a,\alpha} Y^1_{a,\gamma} \quad (2r_T r_V N_v) \quad (9988)$$

$$\tau^2_{\gamma,\alpha} = \sum_{i \in O} W^3_{i,\alpha} Y^2_{i,\gamma} \quad (2r_T r_V N_o) \quad (10001)$$

$$\tau^5_{\gamma,\alpha} = \sum_{i \in O} W^3_{i,\alpha} Y^2_{i,\gamma} \quad (2r_T r_V N_o) \quad (9989)$$

$$\tau^3_{\gamma,\alpha} = \sum_{\beta \in B} X_{\alpha,\beta} \tau^1_{\gamma,\beta} \tau^2_{\gamma,\beta} \quad (3r_T r_V^2) \quad (10002)$$

$$\tau^6_{\gamma,\alpha} = \sum_{\beta \in B} X_{\alpha,\beta} \tau^4_{\gamma,\beta} \tau^5_{\gamma,\beta} \quad (3r_T r_V^2) \quad (9990)$$

$$\tau^4_{\gamma,\alpha} = \sum_{\delta \in A} Z_{\delta,\gamma} \tau^3_{\delta,\alpha} \quad (2r_T^2 r_V) \quad (10003)$$

$$\tau^7_{\gamma,\alpha} = \sum_{\delta \in A} Z_{\delta,\gamma} \tau^6_{\delta,\alpha} \quad (2r_T^2 r_V) \quad (9991)$$

$$\tau^5_{\gamma,\alpha} = \sum_{a \in V} W^2_{a,\alpha} Y^3_{a,\gamma} \quad (2r_T r_V N_v) \quad (10004)$$

$$\tau^8_{\gamma,\alpha} = \sum_{a \in V} W^2_{a,\alpha} Y^3_{a,\gamma} \quad (2r_T r_V N_v) \quad (9992)$$

$$\tau^6_{\gamma,i} = \sum_{\alpha \in B} W^1_{i,\alpha} \tau^4_{\gamma,\alpha} \tau^5_{\gamma,\alpha} \quad (3r_T r_V N_o) \quad (10005)$$

$$\tau^9_{\gamma,i} = \sum_{\alpha \in B} W^1_{i,\alpha} \tau^7_{\gamma,\alpha} \tau^8_{\gamma,\alpha} \quad (3r_T r_V N_o) \quad (9993)$$

$$\tau^7_{i,j} = \sum_{\gamma \in A} Y^4_{j,\gamma} \tau^6_{\gamma,i} \quad (2r_T N_o^2) \quad (10006)$$

$$\tau^{10}_{i,j} = \sum_{\gamma \in A} Y^4_{j,\gamma} \tau^9_{\gamma,i} \quad (2r_T N_o^2) \quad (9994)$$

$$\tau^8_{\gamma,i} = \sum_{j \in O} Y^2_{j,\gamma} \tau^7_{j,i} \quad (2r_T N_o^2) \quad (10007)$$

$$\tau^{11}_{\gamma,i} = \sum_{j \in O} Y^4_{j,\gamma} \tau^{10}_{j,i} \quad (2r_T N_o^2) \quad (9995)$$

$$\tau^9_{\gamma,\delta,w} = \sum_{i \in O} {}^2D^2_{i,w} Y^{2,*}_{i,\delta} \tau^8_{\gamma,i} \quad (3r_D r_T^2 N_o) \quad (10008)$$

$$\tau^{10}_{\gamma,\delta,w} = \sum_{a \in V} {}^2D^1_{a,w} Y^1_{a,\gamma} Y^{1,*}_{a,\delta} \quad (3r_D r_T^2 N_v) \quad (10009)$$

$$\tau^{12}_{\gamma,\delta,w} = \sum_{i \in O} {}^2D^4_{i,w} Y^{4,*}_{i,\delta} \tau^{11}_{\gamma,i} \quad (3r_D r_T^2 N_o) \quad (9996)$$

$$\tau^{11}_{\gamma,\delta,w} = \sum_{\epsilon \in A} Z^*_{\epsilon,\delta} \tau^{10}_{\gamma,\epsilon,w} \tau^9_{\gamma,\epsilon,w} \quad (3r_D r_T^3) \quad (10010)$$

$${}^2R^3_{a,\gamma} \leftarrow - \sum_{\delta \in A} \sum_{w \in D} \frac{1}{2} {}^2D^3_{a,w} Y^3_{a,\delta} \tau^{12}_{\delta,\gamma,w} \tau^3_{\delta,\gamma,w} \quad (4r_D r_T^2 N_v) \quad (9997)$$

$$\tau^{12}_{\gamma,\delta,w} = \sum_{\epsilon \in A} Z_{\epsilon,\gamma} \tau^{11}_{\epsilon,\delta,w} \quad (2r_D r_T^3) \quad (10011)$$

Raw expression

$${}^2R^3_{b,\zeta} \leftarrow - \sum_{\gamma \in A} \sum_{i \in O} \sum_{j \in O} \sum_{k \in O} \sum_{l \in O} \sum_{a \in V} \sum_{c \in V} \sum_{d \in V} \frac{1}{2} Y^{1,*}_{a,\gamma} Y^{2,*}_{i,\gamma} Z^*_{\gamma,\zeta} Y^{4,*}_{j,\zeta} {}^2D^{a,i,b,j} {}^2T_{a,i,d,j} {}^2T_{c,k,b,l} V_{k,c,l,d} \quad (9998)$$

$${}^2R^3_{a,\gamma} \leftarrow - \sum_{\delta \in A} \sum_{w \in D} \frac{1}{2} {}^2D^3_{a,w} Y^3_{a,\delta} \tau^0_{\delta,\gamma,w} \tau^{12}_{\delta,\gamma,w} \quad (4r_D r_T^2 N_v) \quad (10012)$$

Raw expression

Factorized expression

$$\tau^0_{\gamma,\delta,w} = \sum_{i \in O} {}^2D^4_{i,w} Y^4_{i,\gamma} Y^{4,*}_{i,\delta} \quad (3r_D r_T^2 N_o) \quad (9999)$$

$${}^2R^3_{b,\zeta} \leftarrow - \sum_{\gamma \in A} \sum_{i \in O} \sum_{j \in O} \sum_{k \in O} \sum_{l \in O} \sum_{a \in V} \sum_{c \in V} \sum_{d \in V} \frac{1}{2} Y^{1,*}_{a,\gamma} Y^{2,*}_{i,\gamma} Z^*_{\gamma,\zeta} Y^{4,*}_{j,\zeta} {}^2D^{a,i,b,j} {}^2T_{a,i,d,l} {}^2T_{b,j,c,k} V_{l,c,k,d} \quad (10013)$$

Factorized expression

$$\tau^0_{\gamma,\delta,w} = \sum_{a \in V} {}^2D^1_{a,w} Y^1_{a,\gamma} Y^{1,*}_{a,\delta} \quad (3r_D r_T^2 N_v) \quad (10014)$$

$$\tau^1_{\gamma,\delta,w} = \sum_{i \in O} {}^2D^2_{i,w} Y^2_{i,\gamma} Y^{2,*}_{i,\delta} \quad (3r_D r_T^2 N_o) \quad (10015)$$

$$\tau^2_{\gamma,\delta,w} = \sum_{\epsilon \in A} Z^*_{\epsilon,\delta} \tau^0_{\gamma,\epsilon,w} \tau^1_{\gamma,\epsilon,w} \quad (3r_D r_T^3) \quad (10016)$$

$$\tau^3_{\gamma,\alpha} = \sum_{a \in V} W^2_{a,\alpha} Y^3_{a,\gamma} \quad (2r_T r_V N_v) \quad (10017)$$

$$\tau^4_{\gamma,\alpha,i} = \sum_{\beta \in B} W^1_{i,\beta} X_{\beta,\alpha} \tau^3_{\gamma,\beta} \quad (3r_T r_V^2 N_o) \quad (10018)$$

$$\tau^5_{\gamma,\alpha} = \sum_{i \in O} W^3_{i,\alpha} Y^4_{i,\gamma} \quad (2r_T r_V N_o) \quad (10019)$$

$$\tau^6_{\gamma,\alpha} = \sum_{a \in V} W^4_{a,\alpha} Y^3_{a,\gamma} \quad (2r_T r_V N_v) \quad (10020)$$

$$\tau^7_{\gamma,\delta,i} = \sum_{\alpha \in B} \tau^5_{\gamma,\alpha} \tau^6_{\delta,\alpha} \tau^4_{\gamma,\alpha,i} \quad (3r_T^2 r_V N_o) \quad (10021)$$

$$\tau^8_{\gamma,\delta} = \sum_{i \in O} Y^4_{i,\delta} \tau^7_{\gamma,\delta,i} \quad (2r_T^2 N_o) \quad (10022)$$

$$\tau^9_{\gamma,\delta} = \sum_{\epsilon \in A} Z_{\gamma,\epsilon} \tau^8_{\delta,\epsilon} \quad (2r_T^3) \quad (10023)$$

$$\tau^{10}_{\gamma,\delta} = \sum_{\epsilon \in A} Z_{\gamma,\epsilon} \tau^9_{\delta,\epsilon} \quad (2r_T^3) \quad (10024)$$

$$\tau^{11}_{\gamma,\delta,w} = \sum_{\epsilon \in A} \tau^{10}_{\gamma,\epsilon} \tau^2_{\epsilon,\delta,w} \quad (2r_D r_T^3) \quad (10025)$$

$$\tau^{12}_{\gamma,\delta,w} = \sum_{i \in O} {}^2D^4_{i,w} Y^2_{i,\gamma} Y^{4,*}_{i,\delta} \quad (3r_D r_T^2 N_o) \quad (10026)$$

$${}^2R^3_{a,\gamma} \leftarrow - \sum_{\delta \in A} \sum_{w \in D} \frac{1}{2} {}^2D^3_{a,w} Y^1_{a,\delta} \tau^{11}_{\delta,\gamma,w} \tau^{12}_{\delta,\gamma,w} \quad (4r_D r_T^2 N_v) \quad (10027)$$

Raw expression

$${}^2R^3_{b,\zeta} \leftarrow - \sum_{\gamma \in A} \sum_{i \in O} \sum_{j \in O} \sum_{k \in O} \sum_{l \in O} \sum_{a \in V} \sum_{c \in V} \sum_{d \in V} \frac{1}{2} \quad (10028)$$

$$Y^{1,*}_{a,\gamma} Y^{2,*}_{i,\gamma} Z^*_{\gamma,\zeta} Y^{4,*}_{j,\zeta} {}^2D^{a,i,b,j} {}^2T_{a,i,d,l} {}^2T_{b,k,c,j} V_{l,d,k,c}$$

Factorized expression

$$\tau^0_{\gamma,\delta,w} = \sum_{i \in O} {}^2D^4_{i,w} Y^4_{i,\gamma} Y^{4,*}_{i,\delta} \quad (3r_D r_T^2 N_o) \quad (10029)$$

$$\tau^1_{\gamma,\delta,w} = \sum_{a \in V} {}^2D^1_{a,w} Y^1_{a,\gamma} Y^{1,*}_{a,\delta} \quad (3r_D r_T^2 N_v) \quad (10030)$$

$$\tau^2_{\gamma,\delta,w} = \sum_{i \in O} {}^2D^2_{i,w} Y^2_{i,\gamma} Y^{2,*}_{i,\delta} \quad (3r_D r_T^2 N_o) \quad (10031)$$

$$\tau^3_{\gamma,\delta,w} = \sum_{\epsilon \in A} Z^*_{\epsilon,\delta} \tau^1_{\gamma,\epsilon,w} \tau^2_{\gamma,\epsilon,w} \quad (3r_D r_T^3) \quad (10032)$$

$$\tau^4_{\gamma,\delta,w} = \sum_{\epsilon \in A} Z_{\epsilon,\gamma} \tau^3_{\epsilon,\delta,w} \quad (2r_D r_T^3) \quad (10033)$$

$$\tau^5_{\gamma,\alpha} = \sum_{i \in O} W^1_{i,\alpha} Y^2_{i,\gamma} \quad (2r_T r_V N_o) \quad (10034)$$

$$\tau^6_{\gamma,\alpha} = \sum_{a \in V} W^4_{a,\alpha} Y^3_{a,\gamma} \quad (2r_T r_V N_v) \quad (10035)$$

$$\tau^7_{\gamma,\alpha} = \sum_{i \in O} W^3_{i,\alpha} Y^4_{i,\gamma} \quad (2r_T r_V N_o) \quad (10036)$$

$$\tau^8_{\gamma,\alpha} = \sum_{\beta \in B} X_{\alpha,\beta} \tau^6_{\gamma,\beta} \tau^7_{\gamma,\beta} \quad (3r_T r_V^2) \quad (10037)$$

$$\tau^9_{\gamma,\alpha} = \sum_{\delta \in A} Z_{\gamma,\delta} \tau^8_{\delta,\alpha} \quad (2r_T^2 r_V) \quad (10038)$$

$$\tau^{10}_{\gamma,a} = \sum_{\alpha \in B} W^2_{a,\alpha} \tau^5_{\gamma,\alpha} \tau^9_{\gamma,\alpha} \quad (3r_T r_V N_v) \quad (10039)$$

$$\tau^{11}_{a,b} = \sum_{\gamma \in A} Y^1_{b,\gamma} \tau^{10}_{\gamma,a} \quad (2r_T N_v^2) \quad (10040)$$

$$\tau^{12}_{\gamma,a} = \sum_{b \in V} Y^3_{b,\gamma} \tau^{11}_{b,a} \quad (2r_T N_v^2) \quad (10041)$$

$$\tau^{10}_{\gamma,\delta,i} = \sum_{\epsilon \in A} Z_{\gamma,\epsilon} Y^4_{i,\epsilon} \tau^9_{\gamma,\delta,\epsilon} \quad (3r_T^3 N_o) \quad (10054)$$

$${}^2R^3_{a,\gamma} \leftarrow - \sum_{\delta \in A} \sum_{w \in D} \frac{1}{2} {}^2D^3_{a,w} \tau^{12}_{\delta,a} \tau^0_{\delta,\gamma,w} \tau^4_{\delta,\gamma,w} \quad (4r_D r_T^2 N_v^{11}) \quad (10042)$$

$$\tau^{\pi^{11}}_{\gamma,\delta,w} = \sum_{\epsilon \in A} \sum_{i \in O} {}^2D^4_{i,w} Y^{4,*}_{i,\delta} \tau^{10}_{\gamma,\epsilon,i} \tau^2_{\epsilon,\delta,w} \quad (4r_D r_T^3 N_o) \quad (10055)$$

Raw expression

$${}^2R^3_{b,\zeta} \leftarrow - \sum_{\gamma \in A} \sum_{i \in O} \sum_{j \in O} \sum_{k \in O} \sum_{l \in O} \sum_{a \in V} \sum_{c \in V} \sum_{d \in V} \frac{1}{2} \quad (10043)$$

$$Y^{1,*}_{a,\gamma} Y^{2,*}_{i,\gamma} Z^*_{\gamma,\zeta} Y^{4,*}_{j,\zeta}$$

$${}^2D^{a,i,b,j} {}^2T_{a,i,d,l} {}^2T_{c,j,b,k} V_{l,d,k,c}$$

Factorized expression

$$\tau^0_{\gamma,\delta,w} = \sum_{a \in V} {}^2D^1_{a,w} Y^1_{a,\gamma} Y^{1,*}_{a,\delta} \quad (3r_D r_T^2 N_v) \quad (10044)$$

$$\tau^1_{\gamma,\delta,w} = \sum_{i \in O} {}^2D^2_{i,w} Y^2_{i,\gamma} Y^{2,*}_{i,\delta} \quad (3r_D r_T^2 N_o) \quad (10045)$$

$$\tau^2_{\gamma,\delta,w} = \sum_{\epsilon \in A} Z^*_{\epsilon,\delta} \tau^0_{\gamma,\epsilon,w} \tau^1_{\gamma,\epsilon,w} \quad (3r_D r_T^3) \quad (10046)$$

$$\tau^3_{\gamma,\alpha} = \sum_{a \in V} W^2_{a,\alpha} Y^3_{a,\gamma} \quad (2r_T r_V N_v) \quad (10047)$$

$$\tau^4_{\gamma,\alpha} = \sum_{i \in O} W^1_{i,\alpha} Y^4_{i,\gamma} \quad (2r_T r_V N_o) \quad (10048)$$

$$\tau^5_{\gamma,\alpha} = \sum_{\beta \in B} X_{\beta,\alpha} \tau^3_{\gamma,\beta} \tau^4_{\gamma,\beta} \quad (3r_T r_V^2) \quad (10049)$$

$$\tau^6_{\gamma,\alpha} = \sum_{\delta \in A} Z_{\gamma,\delta} \tau^5_{\delta,\alpha} \quad (2r_T^2 r_V) \quad (10050)$$

$$\tau^7_{\gamma,\alpha} = \sum_{a \in V} W^4_{a,\alpha} Y^3_{a,\gamma} \quad (2r_T r_V N_v) \quad (10051)$$

$$\tau^8_{\gamma,\delta,i} = \sum_{\alpha \in B} W^3_{i,\alpha} \tau^6_{\gamma,\alpha} \tau^7_{\delta,\alpha} \quad (3r_T^2 r_V N_o) \quad (10052)$$

$$\tau^9_{\gamma,\delta,\epsilon} = \sum_{i \in O} Y^2_{i,\gamma} \tau^8_{\delta,\epsilon,i} \quad (2r_T^3 N_o) \quad (10053)$$

$${}^2R^3_{a,\gamma} \leftarrow - \sum_{\delta \in A} \sum_{w \in D} \frac{1}{2} {}^2D^3_{a,w} Y^1_{a,\delta} \tau^{11}_{\delta,\gamma,w} \quad (3r_D r_T^2 N_v) \quad (10056)$$

Raw expression

$${}^2R^3_{b,\zeta} \leftarrow - \sum_{\gamma \in A} \sum_{i \in O} \sum_{j \in O} \sum_{k \in O} \sum_{l \in O} \sum_{a \in V} \sum_{c \in V} \sum_{d \in V} \frac{1}{2} \quad (10057)$$

$$Y^{1,*}_{a,\gamma} Y^{2,*}_{i,\gamma} Z^*_{\gamma,\zeta} Y^{4,*}_{j,\zeta}$$

$${}^2D^{a,i,b,j} {}^2T_{a,i,d,l} {}^2T_{c,k,b,j} V_{l,c,k,d}$$

Factorized expression

$$\tau^0_{\gamma,\delta,w} = \sum_{a \in V} {}^2D^1_{a,w} Y^1_{a,\gamma} Y^{1,*}_{a,\delta} \quad (3r_D r_T^2 N_v) \quad (10058)$$

$$\tau^1_{\gamma,\alpha} = \sum_{a \in V} W^4_{a,\alpha} Y^3_{a,\gamma} \quad (2r_T r_V N_v) \quad (10059)$$

$$\tau^2_{\gamma,\alpha} = \sum_{i \in O} W^3_{i,\alpha} Y^4_{i,\gamma} \quad (2r_T r_V N_o) \quad (10060)$$

$$\tau^3_{\gamma,\alpha} = \sum_{\beta \in B} X_{\alpha,\beta} \tau^1_{\gamma,\beta} \tau^2_{\gamma,\beta} \quad (3r_T r_V^2) \quad (10061)$$

$$\tau^4_{\gamma,\alpha} = \sum_{\delta \in A} Z_{\gamma,\delta} \tau^3_{\delta,\alpha} \quad (2r_T^2 r_V) \quad (10062)$$

$$\tau^5_{\gamma,\alpha} = \sum_{a \in V} W^2_{a,\alpha} Y^3_{a,\gamma} \quad (2r_T r_V N_v) \quad (10063)$$

$$\tau^6_{\gamma,\delta,i} = \sum_{\alpha \in B} W^1_{i,\alpha} \tau^4_{\gamma,\alpha} \tau^5_{\delta,\alpha} \quad (3r_T^2 r_V N_o) \quad (10064)$$

$$\tau^7_{\gamma,\delta,\epsilon} = \sum_{i \in O} Y^2_{i,\gamma} Z_{\gamma,\epsilon} \tau^6_{\delta,\epsilon,i} \quad (3r_T^3 N_o) \quad (10065)$$

$$\tau^8_{\gamma,\delta,i} = \sum_{\epsilon \in A} Y^4_{i,\epsilon} \tau^7_{\gamma,\delta,\epsilon} \quad (2r_T^3 N_o) \quad (10066)$$

$$\tau_{\gamma,\delta,w}^9 = \sum_{\epsilon \in A} \sum_{i \in O} {}^2D_{i,w}^2 Y_{i,\delta}^{2,*} \tau_{\epsilon,\delta,w}^0 \tau_{\epsilon,\gamma,i}^8 \quad (4r_D r_T^3 N_o) \quad (10067)$$

$$\tau_{\gamma,\delta,w}^{10} = \sum_{\epsilon \in A} Z_{\epsilon,\delta}^* \tau_{\gamma,\epsilon,w}^9 \quad (2r_D r_T^3) \quad (10068)$$

$$\tau_{\gamma,\delta,w}^{11} = \sum_{i \in O} {}^2D_{i,w}^4 Y_{i,\gamma}^2 Y_{i,\delta}^{4,*} \quad (3r_D r_T^2 N_o) \quad (10069)$$

$$\tau_{\gamma,a}^8 = \sum_{b \in V} Y_{b,\gamma}^3 \tau_{b,a}^7 \quad (2r_T N_v^2) \quad (10080)$$

$$\tau_{\gamma,\delta,w}^9 = \sum_{a \in V} {}^2D_{a,w}^1 Y_{a,\delta}^{1,*} \tau_{\gamma,a}^8 \quad (3r_D r_T^2 N_v) \quad (10081)$$

$$\tau_{\gamma,\delta,w}^{10} = \sum_{i \in O} {}^2D_{i,w}^2 Y_{i,\gamma}^4 Y_{i,\delta}^{2,*} \quad (3r_D r_T^2 N_o) \quad (10082)$$

$${}^2R_{a,\gamma}^3 \leftarrow - \sum_{\delta \in A} \sum_{w \in D} \frac{1}{2} {}^2D_{a,w}^3 Y_{a,\delta}^1 \tau_{\delta,\gamma,w}^{10} \tau_{\delta,\gamma,w}^{11} \quad (4r_D r_T^2 N_v^2) \quad (10070)$$

Raw expression

$$\tau_{\gamma,\delta,w}^{12} = \sum_{\epsilon \in A} Z_{\gamma,\epsilon} \tau_{\epsilon,\delta,w}^{11} \quad (2r_D r_T^3) \quad (10084)$$

$${}^2R_{b,\zeta}^3 \leftarrow - \sum_{\gamma \in A} \sum_{i \in O} \sum_{j \in O} \sum_{k \in O} \sum_{l \in O} \sum_{a \in V} \sum_{c \in V} \sum_{d \in V} \frac{1}{2} \quad (10071)$$

$$Y_{a,\gamma}^{1,*} Y_{i,\gamma}^{2,*} Z_{\gamma,\zeta}^* Y_{j,\zeta}^{4,*} {}^2D_{a,i,b,j} {}^2T_{a,k,b,j} {}^2T_{c,i,d,l} V_{k,c,l,d}$$

$${}^2R_{a,\gamma}^3 \leftarrow - \sum_{\delta \in A} \sum_{w \in D} \frac{1}{2} {}^2D_{a,w}^3 Y_{a,\delta}^1 \tau_{\delta,\gamma,w}^0 \tau_{\delta,\gamma,w}^{12} \quad (4r_D r_T^2 N_v) \quad (10085)$$

Factorized expression

Raw expression

$$\tau_{\gamma,\delta,w}^0 = \sum_{i \in O} {}^2D_{i,w}^4 Y_{i,\gamma}^2 Y_{i,\delta}^{4,*} \quad (3r_D r_T^2 N_o) \quad (10072)$$

$$\tau_{\gamma,\alpha}^1 = \sum_{i \in O} W_{i,\alpha}^1 Y_{i,\gamma}^2 \quad (2r_T r_V N_o) \quad (10073)$$

$${}^2R_{b,\zeta}^3 \leftarrow - \sum_{\gamma \in A} \sum_{i \in O} \sum_{j \in O} \sum_{k \in O} \sum_{l \in O} \sum_{a \in V} \sum_{c \in V} \sum_{d \in V} \frac{1}{2} \quad (10086)$$

$$Y_{a,\gamma}^{1,*} Y_{i,\gamma}^{2,*} Z_{\gamma,\zeta}^* Y_{j,\zeta}^{4,*} {}^2D_{a,i,b,j} {}^2T_{a,k,b,j} {}^2T_{c,l,d,i} V_{k,d,l,c}$$

Factorized expression

$$\tau_{\gamma,\alpha}^2 = \sum_{a \in V} W_{a,\alpha}^4 Y_{a,\gamma}^3 \quad (2r_T r_V N_v) \quad (10074)$$

$$\tau_{\gamma,\delta,w}^0 = \sum_{i \in O} {}^2D_{i,w}^4 Y_{i,\gamma}^4 Y_{i,\delta}^{4,*} \quad (3r_D r_T^2 N_o) \quad (10087)$$

$$\tau_{\gamma,\alpha}^3 = \sum_{i \in O} W_{i,\alpha}^3 Y_{i,\gamma}^4 \quad (2r_T r_V N_o) \quad (10075)$$

$$\tau_{\gamma,\delta,w}^1 = \sum_{i \in O} {}^2D_{i,w}^2 Y_{i,\gamma}^2 Y_{i,\delta}^{2,*} \quad (3r_D r_T^2 N_o) \quad (10088)$$

$$\tau_{\gamma,\alpha}^4 = \sum_{\beta \in B} X_{\alpha,\beta} \tau_{\gamma,\beta}^2 \tau_{\gamma,\beta}^3 \quad (3r_T r_V^2) \quad (10076)$$

$$\tau_{\gamma,\alpha}^2 = \sum_{i \in O} W_{i,\alpha}^1 Y_{i,\gamma}^2 \quad (2r_T r_V N_o) \quad (10089)$$

$$\tau_{\gamma,\alpha}^5 = \sum_{\delta \in A} Z_{\gamma,\delta} \tau_{\delta,\alpha}^4 \quad (2r_T^2 r_V) \quad (10077)$$

$$\tau_{\gamma,\alpha}^3 = \sum_{a \in V} W_{a,\alpha}^4 Y_{a,\gamma}^3 \quad (2r_T r_V N_v) \quad (10090)$$

$$\tau_{\gamma,a}^6 = \sum_{\alpha \in B} W_{a,\alpha}^2 \tau_{\gamma,\alpha}^1 \tau_{\gamma,\alpha}^5 \quad (3r_T r_V N_v) \quad (10078)$$

$$\tau_{\gamma,\alpha}^4 = \sum_{i \in O} W_{i,\alpha}^3 Y_{i,\gamma}^4 \quad (2r_T r_V N_o) \quad (10091)$$

$$\tau_{a,b}^7 = \sum_{\gamma \in A} Y_{b,\gamma}^1 \tau_{\gamma,a}^6 \quad (2r_T N_v^2) \quad (10079)$$

$$\tau_{\gamma,\alpha}^5 = \sum_{\beta \in B} X_{\alpha,\beta} \tau_{\gamma,\beta}^3 \tau_{\gamma,\beta}^4 \quad (3r_T r_V^2) \quad (10092)$$

$$\tau_{\gamma,\alpha}^6 = \sum_{\delta \in A} Z_{\gamma,\delta} \tau_{\delta,\alpha}^5 \quad (2r_T^2 r_V) \quad (10093)$$

$$\tau_{\gamma,\delta,w}^4 = \sum_{\epsilon \in A} Z_{\epsilon,\gamma} \tau_{\epsilon,\delta,w}^3 \quad (2r_D r_T^3) \quad (10106)$$

$$\tau_{\gamma,a}^7 = \sum_{\alpha \in B} W_{a,\alpha}^2 \tau_{\gamma,\alpha}^2 \tau_{\gamma,\alpha}^6 \quad (3r_T r_V N_v) \quad (10094)$$

$$\tau_{\gamma,\alpha}^5 = \sum_{a \in V} W_{a,\alpha}^2 Y_{a,\gamma}^1 \quad (2r_T r_V N_v) \quad (10107)$$

$$\tau_{a,b}^8 = \sum_{\gamma \in A} Y_{b,\gamma}^1 \tau_{\gamma,a}^7 \quad (2r_T N_v^2) \quad (10095)$$

$$\tau_{\gamma,\alpha}^6 = \sum_{i \in O} W_{i,\alpha}^1 Y_{i,\gamma}^2 \quad (2r_T r_V N_o) \quad (10108)$$

$$\tau_{\gamma,a}^9 = \sum_{b \in V} Y_{b,\gamma}^1 \tau_{b,a}^8 \quad (2r_T N_v^2) \quad (10096)$$

$$\tau_{\gamma,\alpha}^7 = \sum_{\beta \in B} X_{\beta,\alpha} \tau_{\gamma,\beta}^5 \tau_{\gamma,\beta}^6 \quad (3r_T r_V^2) \quad (10109)$$

$$\tau_{\gamma,\delta,w}^{10} = \sum_{a \in V} {}^2D_{a,w}^1 Y_{a,\delta}^{1,*} \tau_{\gamma,a}^9 \quad (3r_D r_T^2 N_v) \quad (10097)$$

$$\tau_{\gamma,\alpha}^8 = \sum_{\delta \in A} Z_{\delta,\gamma} \tau_{\delta,\alpha}^7 \quad (2r_T^2 r_V) \quad (10110)$$

$$\tau_{\gamma,\delta,w}^{11} = \sum_{\epsilon \in A} Z_{\epsilon,\delta}^* \tau_{\gamma,\epsilon,w}^1 \tau_{\gamma,\epsilon,w}^{10} \quad (3r_D r_T^3) \quad (10098)$$

$$\tau_{\gamma,\alpha}^9 = \sum_{i \in O} W_{i,\alpha}^3 Y_{i,\gamma}^4 \quad (2r_T r_V N_o) \quad (10111)$$

$$\tau_{\gamma,\delta,w}^{12} = \sum_{\epsilon \in A} Z_{\epsilon,\gamma} \tau_{\epsilon,\delta,w}^{11} \quad (2r_D r_T^3) \quad (10099)$$

$$\tau_{\gamma,a}^{10} = \sum_{\alpha \in B} W_{a,\alpha}^4 \tau_{\gamma,\alpha}^8 \tau_{\gamma,\alpha}^9 \quad (3r_T r_V N_v) \quad (10112)$$

$${}^2R_{a,\gamma}^3 \leftarrow - \sum_{\delta \in A} \sum_{w \in D} \frac{1}{2} {}^2D_{a,w}^3 Y_{a,\delta}^3 \tau_{\delta,\gamma,w}^0 \tau_{\delta,\gamma,w}^{12} \quad (4r_D r_T^2 N_v) \quad (10100)$$

$$\tau_{\gamma,\delta}^{11} = \sum_{a \in V} Y_{a,\delta}^3 \tau_{\gamma,a}^{10} \quad (2r_T^2 N_v) \quad (10113)$$

Raw expression

$$\tau_{\gamma,a}^{12} = \sum_{\delta \in A} Y_{a,\delta}^3 \tau_{\delta,\gamma}^{11} \quad (2r_T^2 N_v) \quad (10114)$$

$${}^2R_{b,\zeta}^3 \leftarrow - \sum_{\gamma \in A} \sum_{i \in O} \sum_{j \in O} \sum_{k \in O} \sum_{l \in O} \sum_{a \in V} \sum_{c \in V} \sum_{d \in V} \frac{1}{2} \quad (10101)$$

$$Y_{a,\gamma}^{1,*} Y_{i,\gamma}^{2,*} Z_{\gamma,\zeta}^* Y_{j,\zeta}^{4,*} {}^2D_{a,i,b,j} {}^2T_{a,k,d,l} {}^2T_{b,j,c,i} V_{k,c,l,d}$$

$${}^2R_{a,\gamma}^3 \leftarrow - \sum_{\delta \in A} \sum_{w \in D} \frac{1}{2} {}^2D_{a,w}^3 \tau_{\delta,a}^{12} \tau_{\delta,\gamma,w}^0 \tau_{\delta,\gamma,w}^4 \quad (4r_D r_T^2 N_v) \quad (10115)$$

Factorized expression

Raw expression

$$\tau_{\gamma,\delta,w}^0 = \sum_{i \in O} {}^2D_{i,w}^4 Y_{i,\gamma}^4 Y_{i,\delta}^{4,*} \quad (3r_D r_T^2 N_o) \quad (10102)$$

$${}^2R_{b,\zeta}^3 \leftarrow - \sum_{\gamma \in A} \sum_{i \in O} \sum_{j \in O} \sum_{k \in O} \sum_{l \in O} \sum_{a \in V} \sum_{c \in V} \sum_{d \in V} \frac{1}{2} \quad (10116)$$

$$Y_{a,\gamma}^{1,*} Y_{i,\gamma}^{2,*} Z_{\gamma,\zeta}^* Y_{j,\zeta}^{4,*} {}^2D_{a,i,b,j} {}^2T_{a,k,d,l} {}^2T_{c,i,b,j} V_{k,c,l,d}$$

$$\tau_{\gamma,\delta,w}^1 = \sum_{a \in V} {}^2D_{a,w}^1 Y_{a,\gamma}^1 Y_{a,\delta}^{1,*} \quad (3r_D r_T^2 N_v) \quad (10103)$$

Factorized expression

$$\tau_{\gamma,\delta,w}^2 = \sum_{i \in O} {}^2D_{i,w}^2 Y_{i,\gamma}^2 Y_{i,\delta}^{2,*} \quad (3r_D r_T^2 N_o) \quad (10104)$$

$$\tau_{\gamma,\delta,w}^0 = \sum_{a \in V} {}^2D_{a,w}^1 Y_{a,\gamma}^1 Y_{a,\delta}^{1,*} \quad (3r_D r_T^2 N_v) \quad (10117)$$

$$\tau_{\gamma,\delta,w}^3 = \sum_{\epsilon \in A} Z_{\epsilon,\delta}^* \tau_{\gamma,\epsilon,w}^1 \tau_{\gamma,\epsilon,w}^2 \quad (3r_D r_T^3) \quad (10105)$$

$$\tau_{\gamma,\delta,w}^1 = \sum_{i \in O} {}^2D_{i,w}^2 Y_{i,\gamma}^2 Y_{i,\delta}^{2,*} \quad (3r_D r_T^2 N_o) \quad (10118)$$

$$\tau_{\gamma,\delta,w}^2 = \sum_{\epsilon \in A} Z_{\epsilon,\delta}^* \tau_{\gamma,\epsilon,w}^0 \tau_{\gamma,\epsilon,w}^1 \quad (3r_D r_T^3) \quad (10119)$$

$$\tau_{\gamma,\alpha}^3 = \sum_{a \in V} W_{a,\alpha}^2 Y_{a,\gamma}^1 \quad (2r_T r_V N_v) \quad (10120)$$

$$\tau_{\gamma,\alpha,i}^4 = \sum_{\beta \in B} W_{i,\beta}^1 X_{\beta,\alpha} \tau_{\gamma,\beta}^3 \quad (3r_T r_V^2 N_o) \quad (10121)$$

$$\tau_{\gamma,\alpha}^5 = \sum_{i \in O} W_{i,\alpha}^3 Y_{i,\gamma}^2 \quad (2r_T r_V N_o) \quad (10122)$$

$$\tau_{\gamma,\alpha}^6 = \sum_{a \in V} W_{a,\alpha}^4 Y_{a,\gamma}^3 \quad (2r_T r_V N_v) \quad (10123)$$

$$\tau_{\gamma,\delta,i}^7 = \sum_{\alpha \in B} \tau_{\gamma,\alpha}^5 \tau_{\delta,\alpha}^6 \tau_{\gamma,\alpha,i}^4 \quad (3r_T^2 r_V N_o) \quad (10124)$$

$$\tau_{\gamma,\delta}^8 = \sum_{i \in O} Y_{i,\delta}^4 \tau_{\gamma,\delta,i}^7 \quad (2r_T^2 N_o) \quad (10125)$$

$$\tau_{\gamma,\delta}^9 = \sum_{\epsilon \in A} Z_{\delta,\epsilon} \tau_{\gamma,\epsilon}^8 \quad (2r_T^3) \quad (10126)$$

$$\tau_{\gamma,\delta}^{10} = \sum_{\epsilon \in A} Z_{\epsilon,\delta} \tau_{\epsilon,\gamma}^9 \quad (2r_T^3) \quad (10127)$$

$$\tau_{\gamma,\delta,w}^{11} = \sum_{\epsilon \in A} \tau_{\epsilon,\gamma}^{10} \tau_{\epsilon,\delta,w}^2 \quad (2r_D r_T^3) \quad (10128)$$

$$\tau_{\gamma,\delta,w}^{12} = \sum_{i \in O} {}^2D_{i,w}^4 Y_{i,\gamma}^4 Y_{i,\delta}^{4,*} \quad (3r_D r_T^2 N_o) \quad (10129)$$

$${}^2R_{a,\gamma}^3 \leftarrow - \sum_{\delta \in A} \sum_{w \in D} \frac{1}{2} {}^2D_{a,w}^3 Y_{a,\delta}^3 \tau_{\delta,\gamma,w}^{11} \tau_{\delta,\gamma,w}^{12} \quad (4r_D r_T^2 N_v) \quad (10130)$$

Raw expression

$${}^2R_{b,\zeta}^3 \leftarrow - \sum_{\gamma \in A} \sum_{i \in O} \sum_{j \in O} \sum_{k \in O} \sum_{l \in O} \sum_{a \in V} \sum_{c \in V} \sum_{d \in V} \frac{1}{2} \quad (10131)$$

$$Y_{a,\gamma}^{1,*} Y_{i,\gamma}^{2,*} Z_{\gamma,\zeta}^* Y_{j,\zeta}^{4,*} {}^2D_{a,i,b,j} {}^2T_{a,l,d,i} {}^2T_{b,j,c,k} V_{l,d,k,c}$$

Factorized expression

$$\tau_{\gamma,\delta,w}^0 = \sum_{a \in V} {}^2D_{a,w}^1 Y_{a,\gamma}^1 Y_{a,\delta}^{1,*} \quad (3r_D r_T^2 N_v) \quad (10132)$$

$$\tau_{\gamma,\delta,w}^1 = \sum_{i \in O} {}^2D_{i,w}^2 Y_{i,\gamma}^2 Y_{i,\delta}^{2,*} \quad (3r_D r_T^2 N_o) \quad (10133)$$

$$\tau_{\gamma,\delta,w}^2 = \sum_{\epsilon \in A} Z_{\epsilon,\delta}^* \tau_{\gamma,\epsilon,w}^0 \tau_{\gamma,\epsilon,w}^1 \quad (3r_D r_T^3) \quad (10134)$$

$$\tau_{\gamma,\alpha}^3 = \sum_{a \in V} W_{a,\alpha}^4 Y_{a,\gamma}^1 \quad (2r_T r_V N_v) \quad (10135)$$

$$\tau_{\gamma,\alpha}^4 = \sum_{a \in V} W_{a,\alpha}^2 Y_{a,\gamma}^3 \quad (2r_T r_V N_v) \quad (10136)$$

$$\tau_{\gamma,\alpha}^5 = \sum_{i \in O} W_{i,\alpha}^1 Y_{i,\gamma}^4 \quad (2r_T r_V N_o) \quad (10137)$$

$$\tau_{\gamma,\alpha}^6 = \sum_{\beta \in B} X_{\beta,\alpha} \tau_{\gamma,\beta}^4 \tau_{\gamma,\beta}^5 \quad (3r_T r_V^2) \quad (10138)$$

$$\tau_{\gamma,\alpha}^7 = \sum_{\delta \in A} Z_{\gamma,\delta} \tau_{\delta,\alpha}^6 \quad (2r_T^2 r_V) \quad (10139)$$

$$\tau_{\gamma,\delta,i}^8 = \sum_{\alpha \in B} W_{i,\alpha}^3 \tau_{\gamma,\alpha}^3 \tau_{\delta,\alpha}^7 \quad (3r_T^2 r_V N_o) \quad (10140)$$

$$\tau_{\gamma,\delta,\epsilon}^9 = \sum_{i \in O} Z_{\gamma,\epsilon} Y_{i,\epsilon}^4 \tau_{\gamma,\delta,i}^8 \quad (3r_T^3 N_o) \quad (10141)$$

$$\tau_{\gamma,\delta,i}^{10} = \sum_{\epsilon \in A} Y_{i,\epsilon}^2 \tau_{\epsilon,\gamma,\delta}^9 \quad (2r_T^3 N_o) \quad (10142)$$

$$\tau_{\gamma,\delta,w}^{11} = \sum_{\epsilon \in A} \sum_{i \in O} {}^2D_{i,w}^4 Y_{i,\delta}^{4,*} \tau_{\epsilon,\gamma,i}^{10} \tau_{\epsilon,\delta,w}^2 \quad (4r_D r_T^3 N_o) \quad (10143)$$

$${}^2R_{a,\gamma}^3 \leftarrow - \sum_{\delta \in A} \sum_{w \in D} \frac{1}{2} {}^2D_{a,w}^3 Y_{a,\delta}^3 \tau_{\delta,\gamma,w}^{11} \quad (3r_D r_T^2 N_v) \quad (10144)$$

Raw expression

$${}^2R^3_{b,\zeta} \leftarrow - \sum_{\gamma \in A} \sum_{i \in O} \sum_{j \in O} \sum_{k \in O} \sum_{l \in O} \sum_{a \in V} \sum_{c \in V} \sum_{d \in V} \frac{1}{2} \quad (10145)$$

$$Y^{1,*}_{a,\gamma} \ Y^{2,*}_{i,\gamma} \ Z^*_{\gamma,\zeta} \ Y^{4,*}_{j,\zeta}$$

$${}^2D^{a,i,b,j} \ {}^2T_{a,l,d,i} \ {}^2T_{c,k,b,j} \ V_{l,d,k,c}$$

Factorized expression

$$\tau^0_{\gamma,\delta,w} = \sum_{a \in V} {}^2D^1_{a,w} Y^1_{a,\gamma} Y^{1,*}_{a,\delta} \quad (3r_D r_T^2 N_v) \quad (10146)$$

$$\tau^1_{\gamma,\alpha} = \sum_{a \in V} W^2_{a,\alpha} Y^3_{a,\gamma} \quad (2r_T r_V N_v) \quad (10147)$$

$$\tau^2_{\gamma,\alpha} = \sum_{a \in V} W^4_{a,\alpha} Y^1_{a,\gamma} \quad (2r_T r_V N_v) \quad (10148)$$

$$\tau^3_{\gamma,\alpha} = \sum_{i \in O} W^3_{i,\alpha} Y^2_{i,\gamma} \quad (2r_T r_V N_o) \quad (10149)$$

$$\tau^4_{\gamma,\alpha} = \sum_{\beta \in B} X_{\alpha,\beta} \tau^2_{\gamma,\beta} \tau^3_{\gamma,\beta} \quad (3r_T r_V^2) \quad (10150)$$

$$\tau^5_{\gamma,\alpha} = \sum_{\delta \in A} Z_{\delta,\gamma} \tau^4_{\delta,\alpha} \quad (2r_T^2 r_V) \quad (10151)$$

$$\tau^6_{\gamma,\delta,i} = \sum_{\alpha \in B} W^1_{i,\alpha} \tau^1_{\delta,\alpha} \tau^5_{\gamma,\alpha} \quad (3r_T^2 r_V N_o) \quad (10152)$$

$$\tau^7_{\gamma,\delta,\epsilon} = \sum_{i \in O} Y^2_{i,\gamma} \tau^6_{\delta,\epsilon,i} \quad (2r_T^3 N_o) \quad (10153)$$

$$\tau^8_{\gamma,\delta,i} = \sum_{\epsilon \in A} Z_{\gamma,\epsilon} Y^4_{i,\epsilon} \tau^7_{\gamma,\delta,\epsilon} \quad (3r_T^3 N_o) \quad (10154)$$

$$\tau^9_{\gamma,\delta,w} = \sum_{\epsilon \in A} \sum_{i \in O} {}^2D^2_{i,w} Y^{2,*}_{i,\delta} \tau^0_{\epsilon,\delta,w} \tau^8_{\epsilon,\gamma,i} \quad (4r_D r_T^3 N_o) \quad (10155)$$

$$\tau^{10}_{\gamma,\delta,w} = \sum_{\epsilon \in A} Z^*_{\epsilon,\delta} \tau^9_{\gamma,\epsilon,w} \quad (2r_D r_T^3) \quad (10156)$$

$$\tau^{11}_{\gamma,\delta,w} = \sum_{i \in O} {}^2D^4_{i,w} Y^4_{i,\gamma} Y^{4,*}_{i,\delta} \quad (3r_D r_T^2 N_o) \quad (10157)$$

$${}^2R^3_{a,\gamma} \leftarrow - \sum_{\delta \in A} \sum_{w \in D} \frac{1}{2} {}^2D^3_{a,w} Y^3_{a,\delta} \tau^{10}_{\delta,\gamma,w} \tau^{11}_{\delta,\gamma,w} \quad (4r_D r_T^2 N_v) \quad (10158)$$

Raw expression

$${}^2R^3_{b,\zeta} \leftarrow - \sum_{\gamma \in A} \sum_{i \in O} \sum_{j \in O} \sum_{k \in O} \sum_{l \in O} \sum_{a \in V} \sum_{c \in V} \sum_{d \in V} \frac{1}{2} \quad (10159)$$

$$Y^{1,*}_{a,\gamma} \ Y^{2,*}_{i,\gamma} \ Z^*_{\gamma,\zeta} \ Y^{4,*}_{j,\zeta}$$

$${}^2D^{a,i,b,j} \ {}^2T_{b,j,a,k} \ {}^2T_{c,i,d,l} \ V_{k,c,l,d}$$

Factorized expression

$$\tau^0_{\gamma,\delta,w} = \sum_{a \in V} {}^2D^1_{a,w} Y^3_{a,\gamma} Y^{1,*}_{a,\delta} \quad (3r_D r_T^2 N_v) \quad (10160)$$

$$\tau^1_{\gamma,\alpha} = \sum_{a \in V} W^4_{a,\alpha} Y^3_{a,\gamma} \quad (2r_T r_V N_v) \quad (10161)$$

$$\tau^2_{\gamma,\alpha} = \sum_{i \in O} W^3_{i,\alpha} Y^4_{i,\gamma} \quad (2r_T r_V N_o) \quad (10162)$$

$$\tau^3_{\gamma,\alpha} = \sum_{\beta \in B} X_{\alpha,\beta} \tau^1_{\gamma,\beta} \tau^2_{\gamma,\beta} \quad (3r_T r_V^2) \quad (10163)$$

$$\tau^4_{\gamma,\alpha} = \sum_{\delta \in A} Z_{\gamma,\delta} \tau^3_{\delta,\alpha} \quad (2r_T^2 r_V) \quad (10164)$$

$$\tau^5_{\gamma,\alpha} = \sum_{a \in V} W^2_{a,\alpha} Y^1_{a,\gamma} \quad (2r_T r_V N_v) \quad (10165)$$

$$\tau^6_{\gamma,\delta,i} = \sum_{\alpha \in B} W^1_{i,\alpha} \tau^4_{\delta,\alpha} \tau^5_{\gamma,\alpha} \quad (3r_T^2 r_V N_o) \quad (10166)$$

$$\tau^7_{\gamma,\delta,\epsilon} = \sum_{i \in O} Z_{\gamma,\epsilon} Y^4_{i,\epsilon} \tau^6_{\gamma,\delta,i} \quad (3r_T^3 N_o) \quad (10167)$$

$$\tau^8_{\gamma,\delta,i} = \sum_{\epsilon \in A} Y^2_{i,\epsilon} \tau^7_{\epsilon,\gamma,\delta} \quad (2r_T^3 N_o) \quad (10168)$$

$$\tau^9_{\gamma,\delta,w} = \sum_{\epsilon \in A} \sum_{i \in O} {}^2D^2_{i,w} Y^{2,*}_{i,\delta} \tau^0_{\epsilon,\delta,w} \tau^8_{\gamma,\epsilon,i} \quad (4r_D r_T^3 N_o) \quad (10169)$$

$$\tau^{10}_{\gamma,\delta,w} = \sum_{\epsilon \in A} Z^*_{\epsilon,\delta} \tau^9_{\gamma,\epsilon,w} \quad (2r_D r_T^3) \quad (10170)$$

$$\tau^{11}_{\gamma,\delta,w} = \sum_{i \in O} {}^2D^4_{i,w} Y^2_{i,\gamma} Y^{4,*}_{i,\delta} \quad (3r_D r_T^2 N_o) \quad (10171)$$

$$\tau^9_{\gamma,i} = \sum_{j \in O} Y^4_{j,\gamma} \tau^8_{j,i} \quad (2r_T N_o^2) \quad (10183)$$

$${}^2R^3_{a,\gamma} \leftarrow - \sum_{\delta \in A} \sum_{w \in D} \frac{1}{2} {}^2D^3_{a,w} Y^1_{a,\delta} \tau^{10}_{\delta,\gamma,w} \tau^{11}_{\delta,\gamma,w} \quad (4r_D r_T^2 N_v) \quad (10172)$$

$$\tau^{10}_{\gamma,\delta,w} = \sum_{i \in O} {}^2D^2_{i,w} Y^{2,*}_{i,\delta} \tau^9_{\gamma,i} \quad (3r_D r_T^2 N_o) \quad (10184)$$

$$\tau^{11}_{\gamma,\delta,w} = \sum_{\epsilon \in A} Z^*_{\epsilon,\delta} \tau^1_{\gamma,\epsilon,w} \tau^{10}_{\gamma,\epsilon,w} \quad (3r_D r_T^3) \quad (10185)$$

Raw expression

$${}^2R^3_{b,\zeta} \leftarrow - \sum_{\gamma \in A} \sum_{i \in O} \sum_{j \in O} \sum_{k \in O} \sum_{l \in O} \sum_{a \in V} \sum_{c \in V} \sum_{d \in V} \frac{1}{2} \quad (10173)$$

$$Y^{1,*}_{a,\gamma} Y^{2,*}_{i,\gamma} Z^*_{\gamma,\zeta} Y^{4,*}_{j,\zeta} \quad (2r_D r_T^3) \quad (10186)$$

$${}^2D^{a,i,b,j} {}^2T_{b,j,a,k} {}^2T_{c,l,d,i} V_{k,d,l,c}$$

$${}^2R^3_{a,\gamma} \leftarrow - \sum_{\delta \in A} \sum_{w \in D} \frac{1}{2} {}^2D^3_{a,w} Y^1_{a,\delta} \tau^0_{\delta,\gamma,w} \tau^{12}_{\delta,\gamma,w} \quad (4r_D r_T^2 N_v) \quad (10187)$$

Factorized expression

$$\tau^0_{\gamma,\delta,w} = \sum_{i \in O} {}^2D^4_{i,w} Y^2_{i,\gamma} Y^{4,*}_{i,\delta} \quad (3r_D r_T^2 N_o) \quad (10174)$$

Raw expression

$$\tau^1_{\gamma,\delta,w} = \sum_{a \in V} {}^2D^1_{a,w} Y^3_{a,\gamma} Y^{1,*}_{a,\delta} \quad (3r_D r_T^2 N_v) \quad (10175)$$

$${}^2R^3_{b,\zeta} \leftarrow - \sum_{\gamma \in A} \sum_{i \in O} \sum_{j \in O} \sum_{k \in O} \sum_{l \in O} \sum_{a \in V} \sum_{c \in V} \sum_{d \in V} \frac{1}{2} \quad (10188)$$

$$Y^{1,*}_{a,\gamma} Y^{2,*}_{i,\gamma} Z^*_{\gamma,\zeta} Y^{4,*}_{j,\zeta} \quad (2r_D r_T^3)$$

$${}^2D^{a,i,b,j} {}^2T_{b,j,c,i} {}^2T_{d,k,a,l} V_{k,d,l,c}$$

Factorized expression

$$\tau^2_{\gamma,\alpha} = \sum_{a \in V} W^2_{a,\alpha} Y^1_{a,\gamma} \quad (2r_T r_V N_v) \quad (10176)$$

$$\tau^0_{\gamma,\delta,w} = \sum_{i \in O} {}^2D^4_{i,w} Y^2_{i,\gamma} Y^{4,*}_{i,\delta} \quad (3r_D r_T^2 N_o) \quad (10189)$$

$$\tau^3_{\gamma,\alpha} = \sum_{a \in V} W^4_{a,\alpha} Y^3_{a,\gamma} \quad (2r_T r_V N_v) \quad (10177)$$

$$\tau^1_{\gamma,\alpha} = \sum_{a \in V} W^2_{a,\alpha} Y^1_{a,\gamma} \quad (2r_T r_V N_v) \quad (10190)$$

$$\tau^4_{\gamma,\alpha} = \sum_{i \in O} W^3_{i,\alpha} Y^4_{i,\gamma} \quad (2r_T r_V N_o) \quad (10178)$$

$$\tau^2_{\gamma,\alpha} = \sum_{i \in O} W^1_{i,\alpha} Y^2_{i,\gamma} \quad (2r_T r_V N_o) \quad (10191)$$

$$\tau^5_{\gamma,\alpha} = \sum_{\beta \in B} X_{\alpha,\beta} \tau^3_{\gamma,\beta} \tau^4_{\gamma,\beta} \quad (3r_T r_V^2) \quad (10179)$$

$$\tau^3_{\gamma,\alpha} = \sum_{\beta \in B} X_{\beta,\alpha} \tau^1_{\gamma,\beta} \tau^2_{\gamma,\beta} \quad (3r_T r_V^2) \quad (10192)$$

$$\tau^6_{\gamma,\alpha} = \sum_{\delta \in A} Z_{\gamma,\delta} \tau^5_{\delta,\alpha} \quad (2r_T^2 r_V) \quad (10180)$$

$$\tau^4_{\gamma,\alpha} = \sum_{\delta \in A} Z_{\delta,\gamma} \tau^3_{\delta,\alpha} \quad (2r_T^2 r_V) \quad (10193)$$

$$\tau^7_{\gamma,i} = \sum_{\alpha \in B} W^1_{i,\alpha} \tau^2_{\gamma,\alpha} \tau^6_{\gamma,\alpha} \quad (3r_T r_V N_o) \quad (10181)$$

$$\tau^5_{\gamma,\alpha} = \sum_{i \in O} W^3_{i,\alpha} Y^4_{i,\gamma} \quad (2r_T r_V N_o) \quad (10194)$$

$$\tau^8_{i,j} = \sum_{\gamma \in A} Y^2_{j,\gamma} \tau^7_{\gamma,i} \quad (2r_T N_o^2) \quad (10182)$$

$$\tau^6_{\gamma,a} = \sum_{\alpha \in B} W^4_{a,\alpha} \tau^4_{\gamma,\alpha} \tau^5_{\gamma,\alpha} \quad (3r_T r_V N_v) \quad (10195)$$



$$\tau^7_{\gamma,\delta} = \sum_{a \in V} Y^3_{a,\delta} \tau^6_{\gamma,a} \quad (2r_T^2 N_v) \quad (10196)$$

$$\tau^8_{\gamma,a} = \sum_{\delta \in A} Y^3_{a,\delta} \tau^7_{\delta,\gamma} \quad (2r_T^2 N_v) \quad (10197)$$

$$\tau^9_{\gamma,\delta,w} = \sum_{a \in V} {}^2D^1_{a,w} Y^{1,*}_{a,\delta} \tau^8_{\gamma,a} \quad (3r_D r_T^2 N_v) \quad (10198)$$

$$\tau^{10}_{\gamma,\delta,w} = \sum_{i \in O} {}^2D^2_{i,w} Y^4_{i,\gamma} Y^{2,*}_{i,\delta} \quad (3r_D r_T^2 N_o) \quad (10199)$$

$$\tau^{11}_{\gamma,\delta,w} = \sum_{\epsilon \in A} Z^*_{\epsilon,\delta} \tau^{10}_{\gamma,\epsilon,w} \tau^9_{\gamma,\epsilon,w} \quad (3r_D r_T^3) \quad (10200)$$

$$\tau^{12}_{\gamma,\delta,w} = \sum_{\epsilon \in A} Z_{\gamma,\epsilon} \tau^{11}_{\epsilon,\delta,w} \quad (2r_D r_T^3) \quad (10201)$$

$${}^2R^3_{a,\gamma} \leftarrow - \sum_{\delta \in A} \sum_{w \in D} \frac{1}{2} {}^2D^3_{a,w} Y^1_{a,\delta} \tau^0_{\delta,\gamma,w} \tau^{12}_{\delta,\gamma,w} \quad (4r_D r_T^2 N_v) \quad (10202)$$

Raw expression

$${}^2R^3_{b,\zeta} \leftarrow - \sum_{\gamma \in A} \sum_{i \in O} \sum_{j \in O} \sum_{k \in O} \sum_{l \in O} \sum_{a \in V} \sum_{c \in V} \sum_{d \in V} \frac{1}{2} \quad (10203)$$

$$\begin{array}{cccc} Y^{1,*}_{a,\gamma} & Y^{2,*}_{i,\gamma} & Z^*_{\gamma,\zeta} & Y^{4,*}_{j,\zeta} \\ {}^2D^{a,i,b,j} & {}^2T_{b,j,c,k} & {}^2T_{d,i,a,l} & V_{l,d,k,c} \end{array}$$

Factorized expression

$$\tau^0_{\gamma,\delta,w} = \sum_{i \in O} {}^2D^4_{i,w} Y^2_{i,\gamma} Y^{4,*}_{i,\delta} \quad (3r_D r_T^2 N_o) \quad (10204)$$

$$\tau^1_{\gamma,\delta,w} = \sum_{a \in V} {}^2D^1_{a,w} Y^3_{a,\gamma} Y^{1,*}_{a,\delta} \quad (3r_D r_T^2 N_v) \quad (10205)$$

$$\tau^2_{\gamma,\delta,w} = \sum_{i \in O} {}^2D^2_{i,w} Y^4_{i,\gamma} Y^{2,*}_{i,\delta} \quad (3r_D r_T^2 N_o) \quad (10206)$$

$$\tau^3_{\gamma,\delta,w} = \sum_{\epsilon \in A} Z^*_{\epsilon,\delta} \tau^1_{\gamma,\epsilon,w} \tau^2_{\gamma,\epsilon,w} \quad (3r_D r_T^3) \quad (10207)$$

$$\tau^4_{\gamma,\delta,w} = \sum_{\epsilon \in A} Z_{\gamma,\epsilon} \tau^3_{\epsilon,\delta,w} \quad (2r_D r_T^3) \quad (10208)$$

$$\tau^5_{\gamma,\alpha} = \sum_{i \in O} W^1_{i,\alpha} Y^2_{i,\gamma} \quad (2r_T r_V N_o) \quad (10209)$$

$$\tau^6_{\gamma,\alpha} = \sum_{a \in V} W^4_{a,\alpha} Y^3_{a,\gamma} \quad (2r_T r_V N_v) \quad (10210)$$

$$\tau^7_{\gamma,\alpha} = \sum_{i \in O} W^3_{i,\alpha} Y^4_{i,\gamma} \quad (2r_T r_V N_o) \quad (10211)$$

$$\tau^8_{\gamma,\alpha} = \sum_{\beta \in B} X_{\alpha,\beta} \tau^6_{\gamma,\beta} \tau^7_{\gamma,\beta} \quad (3r_T r_V^2) \quad (10212)$$

$$\tau^9_{\gamma,\alpha} = \sum_{\delta \in A} Z_{\gamma,\delta} \tau^8_{\delta,\alpha} \quad (2r_T^2 r_V) \quad (10213)$$

$$\tau^{10}_{\gamma,a} = \sum_{\alpha \in B} W^2_{a,\alpha} \tau^5_{\gamma,\alpha} \tau^9_{\gamma,\alpha} \quad (3r_T r_V N_v) \quad (10214)$$

$$\tau^{11}_{a,b} = \sum_{\gamma \in A} Y^1_{b,\gamma} \tau^{10}_{\gamma,a} \quad (2r_T N_v^2) \quad (10215)$$

$$\tau^{12}_{\gamma,a} = \sum_{b \in V} Y^1_{b,\gamma} \tau^{11}_{b,a} \quad (2r_T N_v^2) \quad (10216)$$

$${}^2R^3_{a,\gamma} \leftarrow - \sum_{\delta \in A} \sum_{w \in D} \frac{1}{2} {}^2D^3_{a,w} \tau^{12}_{\delta,a} \tau^0_{\delta,\gamma,w} \tau^4_{\delta,\gamma,w} \quad (4r_D r_T^2 N_v) \quad (10217)$$

Raw expression

$${}^2R^3_{b,\zeta} \leftarrow - \sum_{\gamma \in A} \sum_{i \in O} \sum_{j \in O} \sum_{k \in O} \sum_{l \in O} \sum_{a \in V} \sum_{c \in V} \sum_{d \in V} \frac{1}{2} \quad (10218)$$

$$\begin{array}{cccc} Y^{1,*}_{a,\gamma} & Y^{2,*}_{i,\gamma} & Z^*_{\gamma,\zeta} & Y^{4,*}_{j,\zeta} \\ {}^2D^{a,i,b,j} & {}^2T_{b,j,c,k} & {}^2T_{d,l,a,i} & V_{l,c,k,d} \end{array}$$

Factorized expression

$$\tau^0_{\gamma,\alpha} = \sum_{a \in V} W^2_{a,\alpha} Y^1_{a,\gamma} \quad (2r_T r_V N_v) \quad (10219)$$

$$\tau^1_{\gamma,\alpha} = \sum_{a \in V} W^4_{a,\alpha} Y^3_{a,\gamma} \quad (2r_T r_V N_v) \quad (10220)$$

Factorized expression

$$\tau^2_{\gamma,\alpha} = \sum_{i \in O} W^3_{i,\alpha} Y^4_{i,\gamma} \quad (2r_T r_V N_o) \quad (10221)$$

$$\tau^3_{\gamma,\alpha} = \sum_{\beta \in B} X_{\alpha,\beta} \tau^1_{\gamma,\beta} \tau^2_{\gamma,\beta} \quad (3r_T r_V^2) \quad (10222)$$

$$\tau^4_{\gamma,\alpha} = \sum_{\delta \in A} Z_{\gamma,\delta} \tau^3_{\delta,\alpha} \quad (2r_T^2 r_V) \quad (10223)$$

$$\tau^5_{\gamma,i} = \sum_{\alpha \in B} W^1_{i,\alpha} \tau^0_{\gamma,\alpha} \tau^4_{\gamma,\alpha} \quad (3r_T r_V N_o) \quad (10224)$$

$$\tau^6_{i,j} = \sum_{\gamma \in A} Y^2_{j,\gamma} \tau^5_{\gamma,i} \quad (2r_T N_o^2) \quad (10225)$$

$$\tau^7_{\gamma,i} = \sum_{j \in O} Y^2_{j,\gamma} \tau^6_{j,i} \quad (2r_T N_o^2) \quad (10226)$$

$$\tau^8_{\gamma,\delta,w} = \sum_{i \in O} {}^2D^4_{i,w} Y^{4,*}_{i,\delta} \tau^7_{\gamma,i} \quad (3r_D r_T^2 N_o) \quad (10227)$$

$$\tau^9_{\gamma,\delta,w} = \sum_{a \in V} {}^2D^1_{a,w} Y^3_{a,\gamma} Y^{1,*}_{a,\delta} \quad (3r_D r_T^2 N_v) \quad (10228)$$

$$\tau^{10}_{\gamma,\delta,w} = \sum_{i \in O} {}^2D^2_{i,w} Y^4_{i,\gamma} Y^{2,*}_{i,\delta} \quad (3r_D r_T^2 N_o) \quad (10229)$$

$$\tau^{11}_{\gamma,\delta,w} = \sum_{\epsilon \in A} Z^*_{\epsilon,\delta} \tau^{10}_{\gamma,\epsilon,w} \tau^9_{\gamma,\epsilon,w} \quad (3r_D r_T^3) \quad (10230)$$

$$\tau^{12}_{\gamma,\delta,w} = \sum_{\epsilon \in A} Z_{\gamma,\epsilon} \tau^{11}_{\epsilon,\delta,w} \quad (2r_D r_T^3) \quad (10231)$$

$${}^2R^3_{a,\gamma} \leftarrow - \sum_{\delta \in A} \sum_{w \in D} \frac{1}{2} {}^2D^3_{a,w} Y^1_{a,\delta} \tau^{12}_{\delta,\gamma,w} \tau^8_{\delta,\gamma,w} \quad (4r_D r_T^2 N_{\mathfrak{A}}) \quad (10232)$$

Raw expression

$${}^2R^3_{b,\zeta} \leftarrow - \sum_{\gamma \in A} \sum_{i \in O} \sum_{j \in O} \sum_{k \in O} \sum_{l \in O} \sum_{a \in V} \sum_{c \in V} \sum_{d \in V} \frac{1}{2} \quad (10233)$$

$$Y^{1,*}_{a,\gamma} Y^{2,*}_{i,\gamma} Z^*_{\gamma,\zeta} Y^{4,*}_{j,\zeta} {}^2D^{a,i,b,j} {}^2T_{b,k,a,i} {}^2T_{c,j,d,l} V_{k,c,l,d}$$

$$\tau^0_{\gamma,\delta,w} = \sum_{a \in V} {}^2D^1_{a,w} Y^3_{a,\gamma} Y^{1,*}_{a,\delta} \quad (3r_D r_T^2 N_v) \quad (10234)$$

$$\tau^1_{\gamma,\delta,w} = \sum_{i \in O} {}^2D^2_{i,w} Y^4_{i,\gamma} Y^{2,*}_{i,\delta} \quad (3r_D r_T^2 N_o) \quad (10235)$$

$$\tau^2_{\gamma,\delta,w} = \sum_{\epsilon \in A} Z^*_{\epsilon,\delta} \tau^0_{\gamma,\epsilon,w} \tau^1_{\gamma,\epsilon,w} \quad (3r_D r_T^3) \quad (10236)$$

$$\tau^3_{\gamma,\alpha} = \sum_{a \in V} W^4_{a,\alpha} Y^3_{a,\gamma} \quad (2r_T r_V N_v) \quad (10237)$$

$$\tau^4_{\gamma,\alpha} = \sum_{a \in V} W^2_{a,\alpha} Y^1_{a,\gamma} \quad (2r_T r_V N_v) \quad (10238)$$

$$\tau^5_{\gamma,\alpha} = \sum_{i \in O} W^1_{i,\alpha} Y^2_{i,\gamma} \quad (2r_T r_V N_o) \quad (10239)$$

$$\tau^6_{\gamma,\alpha} = \sum_{\beta \in B} X_{\beta,\alpha} \tau^4_{\gamma,\beta} \tau^5_{\gamma,\beta} \quad (3r_T r_V^2) \quad (10240)$$

$$\tau^7_{\gamma,\alpha} = \sum_{\delta \in A} Z_{\delta,\gamma} \tau^6_{\delta,\alpha} \quad (2r_T^2 r_V) \quad (10241)$$

$$\tau^8_{\gamma,\delta,i} = \sum_{\alpha \in B} W^3_{i,\alpha} \tau^3_{\delta,\alpha} \tau^7_{\gamma,\alpha} \quad (3r_T^2 r_V N_o) \quad (10242)$$

$$\tau^9_{\gamma,\delta,\epsilon} = \sum_{i \in O} Y^2_{i,\gamma} \tau^8_{\delta,\epsilon,i} \quad (2r_T^3 N_o) \quad (10243)$$

$$\tau^{10}_{\gamma,\delta,i} = \sum_{\epsilon \in A} Z_{\gamma,\epsilon} Y^4_{i,\epsilon} \tau^9_{\gamma,\delta,\epsilon} \quad (3r_T^3 N_o) \quad (10244)$$

$$\tau^{11}_{\gamma,\delta,w} = \sum_{\epsilon \in A} \sum_{i \in O} {}^2D^4_{i,w} Y^{4,*}_{i,\delta} \tau^{10}_{\gamma,\epsilon,i} \tau^2_{\epsilon,\delta,w} \quad (4r_D r_T^3 N_o) \quad (10245)$$

$${}^2R^3_{a,\gamma} \leftarrow - \sum_{\delta \in A} \sum_{w \in D} \frac{1}{2} {}^2D^3_{a,w} Y^1_{a,\delta} \tau^{11}_{\delta,\gamma,w} \quad (3r_D r_T^2 N_v) \quad (10246)$$

Raw expression

$${}^2R^3_{b,\zeta} \leftarrow - \sum_{\gamma \in A} \sum_{i \in O} \sum_{j \in O} \sum_{k \in O} \sum_{l \in O} \sum_{a \in V} \sum_{c \in V} \sum_{d \in V} \frac{1}{2} \quad (10247)$$

$$\begin{matrix} Y^{1,*}_{a,\gamma} & Y^{2,*}_{i,\gamma} & Z^*_{\gamma,\zeta} & Y^{4,*}_{j,\zeta} \\ {}^2D^{a,i,b,j} & {}^2T_{b,k,a,i} & {}^2T_{c,l,d,j} & V_{k,d,l,c} \end{matrix}$$

Factorized expression

$$\tau^0_{\gamma,\delta,w} = \sum_{a \in V} {}^2D^1_{a,w} Y^3_{a,\gamma} Y^{1,*}_{a,\delta} \quad (3r_D r_T^2 N_v) \quad (10248)$$

$$\tau^1_{\gamma,\delta,w} = \sum_{i \in O} {}^2D^2_{i,w} Y^4_{i,\gamma} Y^{2,*}_{i,\delta} \quad (3r_D r_T^2 N_o) \quad (10249)$$

$$\tau^2_{\gamma,\delta,w} = \sum_{\epsilon \in A} Z^*_{\epsilon,\delta} \tau^0_{\gamma,\epsilon,w} \tau^1_{\gamma,\epsilon,w} \quad (3r_D r_T^3) \quad (10250)$$

$$\tau^3_{\gamma,\alpha} = \sum_{a \in V} W^2_{a,\alpha} Y^3_{a,\gamma} \quad (2r_T r_V N_v) \quad (10251)$$

$$\tau^4_{\gamma,\alpha,i} = \sum_{\beta \in B} W^1_{i,\beta} X_{\beta,\alpha} \tau^3_{\gamma,\beta} \quad (3r_T r_V^2 N_o) \quad (10252)$$

$$\tau^5_{\gamma,\alpha} = \sum_{i \in O} W^3_{i,\alpha} Y^4_{i,\gamma} \quad (2r_T r_V N_o) \quad (10253)$$

$$\tau^6_{\gamma,\alpha} = \sum_{a \in V} W^4_{a,\alpha} Y^1_{a,\gamma} \quad (2r_T r_V N_v) \quad (10254)$$

$$\tau^7_{\gamma,\delta,i} = \sum_{\alpha \in B} \tau^5_{\delta,\alpha} \tau^6_{\gamma,\alpha} \tau^4_{\delta,\alpha,i} \quad (3r_T^2 r_V N_o) \quad (10255)$$

$$\tau^8_{\gamma,\delta} = \sum_{i \in O} Y^2_{i,\gamma} \tau^7_{\gamma,\delta,i} \quad (2r_T^2 N_o) \quad (10256)$$

$$\tau^9_{\gamma,\delta} = \sum_{\epsilon \in A} Z_{\delta,\epsilon} \tau^8_{\gamma,\epsilon} \quad (2r_T^3) \quad (10257)$$

$$\tau^{10}_{\gamma,\delta} = \sum_{\epsilon \in A} Z_{\epsilon,\delta} \tau^9_{\epsilon,\gamma} \quad (2r_T^3) \quad (10258)$$

$$\tau^{11}_{\gamma,\delta,w} = \sum_{\epsilon \in A} \tau^{10}_{\gamma,\epsilon} \tau^2_{\epsilon,\delta,w} \quad (2r_D r_T^3) \quad (10259)$$

$$\tau^{12}_{\gamma,\delta,w} = \sum_{i \in O} {}^2D^4_{i,w} Y^2_{i,\gamma} Y^{4,*}_{i,\delta} \quad (3r_D r_T^2 N_o) \quad (10260)$$

$${}^2R^3_{a,\gamma} \leftarrow - \sum_{\delta \in A} \sum_{w \in D} \frac{1}{2} {}^2D^3_{a,w} Y^1_{a,\delta} \tau^{11}_{\delta,\gamma,w} \tau^{12}_{\delta,\gamma,w} \quad (4r_D r_T^2 N_v) \quad (10261)$$

Raw expression

$${}^2R^3_{b,\zeta} \leftarrow - \sum_{\gamma \in A} \sum_{i \in O} \sum_{j \in O} \sum_{k \in O} \sum_{l \in O} \sum_{a \in V} \sum_{c \in V} \sum_{d \in V} \frac{1}{2} \quad (10262)$$

$$\begin{matrix} Y^{1,*}_{a,\gamma} & Y^{2,*}_{i,\gamma} & Z^*_{\gamma,\zeta} & Y^{4,*}_{j,\zeta} \\ {}^2D^{a,i,b,j} & {}^2T_{b,k,c,j} & {}^2T_{d,l,a,i} & V_{l,d,k,c} \end{matrix}$$

Factorized expression

$$\tau^0_{\gamma,\delta,w} = \sum_{i \in O} {}^2D^4_{i,w} Y^2_{i,\gamma} Y^{4,*}_{i,\delta} \quad (3r_D r_T^2 N_o) \quad (10263)$$

$$\tau^1_{\gamma,\delta,w} = \sum_{a \in V} {}^2D^1_{a,w} Y^3_{a,\gamma} Y^{1,*}_{a,\delta} \quad (3r_D r_T^2 N_v) \quad (10264)$$

$$\tau^2_{\gamma,\alpha} = \sum_{a \in V} W^4_{a,\alpha} Y^1_{a,\gamma} \quad (2r_T r_V N_v) \quad (10265)$$

$$\tau^3_{\gamma,\alpha} = \sum_{i \in O} W^3_{i,\alpha} Y^2_{i,\gamma} \quad (2r_T r_V N_o) \quad (10266)$$

$$\tau^4_{\gamma,\alpha} = \sum_{\beta \in B} X_{\alpha,\beta} \tau^2_{\gamma,\beta} \tau^3_{\gamma,\beta} \quad (3r_T r_V^2) \quad (10267)$$

$$\tau^5_{\gamma,\alpha} = \sum_{\delta \in A} Z_{\delta,\gamma} \tau^4_{\delta,\alpha} \quad (2r_T^2 r_V) \quad (10268)$$

$$\tau^6_{\gamma,\alpha} = \sum_{a \in V} W^2_{a,\alpha} Y^3_{a,\gamma} \quad (2r_T r_V N_v) \quad (10269)$$

$$\tau^7_{\gamma,i} = \sum_{\alpha \in B} W^1_{i,\alpha} \tau^5_{\gamma,\alpha} \tau^6_{\gamma,\alpha} \quad (3r_T r_V N_o) \quad (10270)$$

$$\tau^8_{i,j} = \sum_{\gamma \in A} Y^4_{j,\gamma} \tau^7_{\gamma,i} \quad (2r_T N_o^2) \quad (10271)$$

$$\tau_{\gamma,i}^9 = \sum_{j \in O} Y_{j,\gamma}^4 \tau_{j,i}^8 \quad (2r_T N_o^2) \quad (10272)$$

$$\tau_{\gamma,i}^7 = \sum_{j \in O} Y_{j,\gamma}^2 \tau_{j,i}^6 \quad (2r_T N_o^2) \quad (10285)$$

$$\tau_{\gamma,\delta,w}^{10} = \sum_{i \in O} {}^2D_{i,w}^2 Y_{i,\delta}^{2,*} \tau_{\gamma,i}^9 \quad (3r_D r_T^2 N_o) \quad (10273)$$

$$\tau_{\gamma,\delta,w}^8 = \sum_{i \in O} {}^2D_{i,w}^4 Y_{i,\delta}^{4,*} \tau_{\gamma,i}^7 \quad (3r_D r_T^2 N_o) \quad (10286)$$

$$\tau_{\gamma,\delta,w}^{11} = \sum_{\epsilon \in A} Z_{\epsilon,\delta}^* \tau_{\gamma,\epsilon,w}^1 \tau_{\gamma,\epsilon,w}^{10} \quad (3r_D r_T^3) \quad (10274)$$

$$\tau_{\gamma,\delta,w}^9 = \sum_{a \in V} {}^2D_{a,w}^1 Y_{a,\gamma}^3 Y_{a,\delta}^{1,*} \quad (3r_D r_T^2 N_v) \quad (10287)$$

$$\tau_{\gamma,\delta,w}^{12} = \sum_{\epsilon \in A} Z_{\gamma,\epsilon} \tau_{\epsilon,\delta,w}^{11} \quad (2r_D r_T^3) \quad (10275)$$

$$\tau_{\gamma,\delta,w}^{10} = \sum_{i \in O} {}^2D_{i,w}^2 Y_{i,\gamma}^4 Y_{i,\delta}^{2,*} \quad (3r_D r_T^2 N_o) \quad (10288)$$

$${}^2R_{a,\gamma}^3 \leftarrow - \sum_{\delta \in A} \sum_{w \in D} \frac{1}{2} {}^2D_{a,w}^3 Y_{a,\delta}^1 \tau_{\delta,\gamma,w}^0 \tau_{\delta,\gamma,w}^{12} \quad (4r_D r_T^2 N_v) \quad (10276)$$

$$\tau_{\gamma,\delta,w}^{11} = \sum_{\epsilon \in A} Z_{\epsilon,\delta}^* \tau_{\gamma,\epsilon,w}^{10} \tau_{\gamma,\epsilon,w}^9 \quad (3r_D r_T^3) \quad (10289)$$

Raw expression

$${}^2R_{b,\zeta}^3 \leftarrow - \sum_{\gamma \in A} \sum_{i \in O} \sum_{j \in O} \sum_{k \in O} \sum_{l \in O} \sum_{a \in V} \sum_{c \in V} \sum_{d \in V} \frac{1}{2} \quad (10277)$$

$$Y_{a,\gamma}^{1,*} Y_{i,\gamma}^{2,*} Z_{\gamma,\zeta}^* Y_{j,\zeta}^{4,*} {}^2D_{a,i,b,j} {}^2T_{b,k,c,l} {}^2T_{d,j,a,i} V_{k,d,l,c}$$

$$\tau_{\gamma,\delta,w}^{12} = \sum_{\epsilon \in A} Z_{\gamma,\epsilon} \tau_{\epsilon,\delta,w}^{11} \quad (2r_D r_T^3) \quad (10290)$$

$${}^2R_{a,\gamma}^3 \leftarrow - \sum_{\delta \in A} \sum_{w \in D} \frac{1}{2} {}^2D_{a,w}^3 Y_{a,\delta}^1 \tau_{\delta,\gamma,w}^{12} \tau_{\delta,\gamma,w}^8 \quad (4r_D r_T^2 N_v) \quad (10291)$$

Factorized expression

$$\tau_{\gamma,\alpha}^0 = \sum_{a \in V} W_{a,\alpha}^4 Y_{a,\gamma}^1 \quad (2r_T r_V N_v) \quad (10278)$$

Raw expression

$$\tau_{\gamma,\alpha}^1 = \sum_{i \in O} W_{i,\alpha}^3 Y_{i,\gamma}^2 \quad (2r_T r_V N_o) \quad (10279)$$

$${}^2R_{b,\zeta}^3 \leftarrow - \sum_{\gamma \in A} \sum_{i \in O} \sum_{j \in O} \sum_{k \in O} \sum_{l \in O} \sum_{a \in V} \sum_{c \in V} \sum_{d \in V} \frac{1}{2} \quad (10292)$$

$$Y_{a,\gamma}^{1,*} Y_{i,\gamma}^{2,*} Z_{\gamma,\zeta}^* Y_{j,\zeta}^{4,*} {}^2D_{a,i,b,j} {}^2T_{c,i,b,j} {}^2T_{d,k,a,l} V_{k,d,l,c}$$

$$\tau_{\gamma,\alpha}^2 = \sum_{\beta \in B} X_{\alpha,\beta} \tau_{\gamma,\beta}^0 \tau_{\gamma,\beta}^1 \quad (3r_T r_V^2) \quad (10280)$$

Factorized expression

$$\tau_{\gamma,\alpha}^3 = \sum_{\delta \in A} Z_{\delta,\gamma} \tau_{\delta,\alpha}^2 \quad (2r_T^2 r_V) \quad (10281)$$

$$\tau_{\gamma,\delta,w}^0 = \sum_{a \in V} {}^2D_{a,w}^1 Y_{a,\gamma}^3 Y_{a,\delta}^{1,*} \quad (3r_D r_T^2 N_v) \quad (10293)$$

$$\tau_{\gamma,\alpha}^4 = \sum_{a \in V} W_{a,\alpha}^2 Y_{a,\gamma}^3 \quad (2r_T r_V N_v) \quad (10282)$$

$$\tau_{\gamma,\alpha}^1 = \sum_{a \in V} W_{a,\alpha}^2 Y_{a,\gamma}^1 \quad (2r_T r_V N_v) \quad (10294)$$

$$\tau_{\gamma,i}^5 = \sum_{\alpha \in B} W_{i,\alpha}^1 \tau_{\gamma,\alpha}^3 \tau_{\gamma,\alpha}^4 \quad (3r_T r_V N_o) \quad (10283)$$

$$\tau_{\gamma,\alpha}^2 = \sum_{a \in V} W_{a,\alpha}^4 Y_{a,\gamma}^1 \quad (2r_T r_V N_v) \quad (10295)$$

$$\tau_{i,j}^6 = \sum_{\gamma \in A} Y_{j,\gamma}^4 \tau_{\gamma,i}^5 \quad (2r_T N_o^2) \quad (10284)$$

$$\tau_{\gamma,\alpha}^3 = \sum_{i \in O} W_{i,\alpha}^3 Y_{i,\gamma}^2 \quad (2r_T r_V N_o) \quad (10296)$$

$$\tau^4_{\gamma,\alpha} = \sum_{\beta \in B} X_{\alpha,\beta} \tau^2_{\gamma,\beta} \tau^3_{\gamma,\beta} \quad (3r_T r_V^2) \quad (10297)$$

$$\tau^5_{\gamma,\alpha} = \sum_{\delta \in A} Z_{\delta,\gamma} \tau^4_{\delta,\alpha} \quad (2r_T^2 r_V) \quad (10298)$$

$$\tau^6_{\gamma,\delta,i} = \sum_{\alpha \in B} W^1_{i,\alpha} \tau^1_{\gamma,\alpha} \tau^5_{\delta,\alpha} \quad (3r_T^2 r_V N_o) \quad (10299)$$

$$\tau^7_{\gamma,\delta,\epsilon} = \sum_{i \in O} Z_{\gamma,\delta} Y^4_{i,\delta} \tau^6_{\gamma,\epsilon,i} \quad (3r_T^3 N_o) \quad (10300)$$

$$\tau^8_{\gamma,\delta,i} = \sum_{\epsilon \in A} Y^2_{i,\epsilon} \tau^7_{\epsilon,\gamma,\delta} \quad (2r_T^3 N_o) \quad (10301)$$

$$\tau^9_{\gamma,\delta,w} = \sum_{\epsilon \in A} \sum_{i \in O} {}^2D^2_{i,w} Y^{2,*}_{i,\delta} \tau^0_{\epsilon,\delta,w} \tau^8_{\epsilon,\gamma,i} \quad (4r_D r_T^3 N_o) \quad (10302)$$

$$\tau^{10}_{\gamma,\delta,w} = \sum_{\epsilon \in A} Z^*_{\epsilon,\delta} \tau^9_{\gamma,\epsilon,w} \quad (2r_D r_T^3) \quad (10303)$$

$$\tau^{11}_{\gamma,\delta,w} = \sum_{i \in O} {}^2D^4_{i,w} Y^4_{i,\gamma} Y^{4,*}_{i,\delta} \quad (3r_D r_T^2 N_o) \quad (10304)$$

$${}^2R^3_{a,\gamma} \leftarrow - \sum_{\delta \in A} \sum_{w \in D} \frac{1}{2} {}^2D^3_{a,w} Y^3_{a,\delta} \tau^{10}_{\delta,\gamma,w} \tau^{11}_{\delta,\gamma,w} \quad (4r_D r_T^2 N_v) \quad \tau^{11}_{\gamma,\delta,w} = \sum_{\epsilon \in A} \tau^{10}_{\gamma,\epsilon} \tau^2_{\epsilon,\delta,w} \quad (2r_D r_T^3) \quad (10305)$$

Raw expression

$${}^2R^3_{b,\zeta} \leftarrow - \sum_{\gamma \in A} \sum_{i \in O} \sum_{j \in O} \sum_{k \in O} \sum_{l \in O} \sum_{a \in V} \sum_{c \in V} \sum_{d \in V} \frac{1}{2} Y^{1,*}_{a,\gamma} Y^{2,*}_{i,\gamma} Z^*_{\gamma,\zeta} Y^{4,*}_{j,\zeta} {}^2D^{a,i,b,j} {}^2T_{c,j,b,k} {}^2T_{d,l,a,i} V_{l,d,k,c} \quad (10306)$$

Factorized expression

$$\tau^0_{\gamma,\delta,w} = \sum_{a \in V} {}^2D^1_{a,w} Y^3_{a,\gamma} Y^{1,*}_{a,\delta} \quad (3r_D r_T^2 N_v) \quad (10307)$$

$$\tau^1_{\gamma,\delta,w} = \sum_{i \in O} {}^2D^2_{i,w} Y^4_{i,\gamma} Y^{2,*}_{i,\delta} \quad (3r_D r_T^2 N_o) \quad (10308)$$

$$\tau^2_{\gamma,\delta,w} = \sum_{\epsilon \in A} Z^*_{\epsilon,\delta} \tau^0_{\gamma,\epsilon,w} \tau^1_{\gamma,\epsilon,w} \quad (3r_D r_T^3) \quad (10309)$$

$$\tau^3_{\gamma,\alpha} = \sum_{a \in V} W^2_{a,\alpha} Y^1_{a,\gamma} \quad (2r_T r_V N_v) \quad (10310)$$

$$\tau^4_{\gamma,\alpha,i} = \sum_{\beta \in B} W^1_{i,\beta} X_{\beta,\alpha} \tau^3_{\gamma,\beta} \quad (3r_T r_V^2 N_o) \quad (10311)$$

$$\tau^5_{\gamma,\alpha} = \sum_{i \in O} W^3_{i,\alpha} Y^2_{i,\gamma} \quad (2r_T r_V N_o) \quad (10312)$$

$$\tau^6_{\gamma,\alpha} = \sum_{a \in V} W^4_{a,\alpha} Y^1_{a,\gamma} \quad (2r_T r_V N_v) \quad (10313)$$

$$\tau^7_{\gamma,\delta,i} = \sum_{\alpha \in B} \tau^5_{\gamma,\alpha} \tau^6_{\delta,\alpha} \tau^4_{\gamma,\alpha,i} \quad (3r_T^2 r_V N_o) \quad (10314)$$

$$\tau^8_{\gamma,\delta} = \sum_{i \in O} Y^2_{i,\delta} \tau^7_{\gamma,\delta,i} \quad (2r_T^2 N_o) \quad (10315)$$

$$\tau^9_{\gamma,\delta} = \sum_{\epsilon \in A} Z_{\epsilon,\delta} \tau^8_{\gamma,\epsilon} \quad (2r_T^3) \quad (10316)$$

$$\tau^{10}_{\gamma,\delta} = \sum_{\epsilon \in A} Z_{\epsilon,\gamma} \tau^9_{\epsilon,\delta} \quad (2r_T^3) \quad (10317)$$

$$\tau^{12}_{\gamma,\delta,w} = \sum_{i \in O} {}^2D^4_{i,w} Y^4_{i,\gamma} Y^{4,*}_{i,\delta} \quad (3r_D r_T^2 N_o) \quad (10319)$$

$${}^2R^3_{a,\gamma} \leftarrow - \sum_{\delta \in A} \sum_{w \in D} \frac{1}{2} {}^2D^3_{a,w} Y^3_{a,\delta} \tau^{11}_{\delta,\gamma,w} \tau^{12}_{\delta,\gamma,w} \quad (4r_D r_T^2 N_v) \quad (10320)$$

Raw expression

$${}^2R^3_{b,\zeta} \leftarrow - \sum_{\gamma \in A} \sum_{i \in O} \sum_{j \in O} \sum_{k \in O} \sum_{l \in O} \sum_{a \in V} \sum_{c \in V} \sum_{d \in V} \frac{1}{2} Y^{1,*}_{a,\gamma} Y^{2,*}_{i,\gamma} Z^*_{\gamma,\zeta} Y^{4,*}_{j,\zeta} {}^2D^{a,i,b,j} {}^2T_{c,k,b,j} {}^2T_{d,i,a,l} V_{l,d,k,c} \quad (10321)$$

Factorized expression

$$\tau^0_{\gamma,\delta,w} = \sum_{i \in O} {}^2D^4_{i,w} Y^4_{i,\gamma} Y^{4,*}_{i,\delta} \quad (3r_D r_T^2 N_o) \quad (10322)$$

$$\tau^1_{\gamma,\delta,w} = \sum_{i \in O} {}^2D^2_{i,w} Y^2_{i,\gamma} Y^{2,*}_{i,\delta} \quad (3r_D r_T^2 N_o) \quad (10323)$$

$$\tau^2_{\gamma,\alpha} = \sum_{a \in V} W^2_{a,\alpha} Y^1_{a,\gamma} \quad (2r_T r_V N_v) \quad (10324)$$

$$\tau^3_{\gamma,\alpha} = \sum_{i \in O} W^1_{i,\alpha} Y^2_{i,\gamma} \quad (2r_T r_V N_o) \quad (10325)$$

$$\tau^4_{\gamma,\alpha} = \sum_{\beta \in B} X_{\beta,\alpha} \tau^2_{\gamma,\beta} \tau^3_{\gamma,\beta} \quad (3r_T r_V^2) \quad (10326)$$

$$\tau^5_{\gamma,\alpha} = \sum_{\delta \in A} Z_{\delta,\gamma} \tau^4_{\delta,\alpha} \quad (2r_T^2 r_V) \quad (10327)$$

$$\tau^6_{\gamma,\alpha} = \sum_{i \in O} W^3_{i,\alpha} Y^4_{i,\gamma} \quad (2r_T r_V N_o) \quad (10328)$$

$$\tau^7_{\gamma,a} = \sum_{\alpha \in B} W^4_{a,\alpha} \tau^5_{\gamma,\alpha} \tau^6_{\gamma,\alpha} \quad (3r_T r_V N_v) \quad (10329)$$

$$\tau^8_{\gamma,\delta} = \sum_{a \in V} Y^1_{a,\gamma} \tau^7_{\delta,a} \quad (2r_T^2 N_v) \quad (10330)$$

$$\tau^9_{\gamma,a} = \sum_{\delta \in A} Y^3_{a,\delta} \tau^8_{\gamma,\delta} \quad (2r_T^2 N_v) \quad (10331)$$

$$\tau^{10}_{\gamma,\delta,w} = \sum_{a \in V} {}^2D^1_{a,w} Y^{1,*}_{a,\delta} \tau^9_{\gamma,a} \quad (3r_D r_T^2 N_v) \quad (10332)$$

$$\tau^{11}_{\gamma,\delta,w} = \sum_{\epsilon \in A} Z^*_{\epsilon,\delta} \tau^1_{\gamma,\epsilon,w} \tau^{10}_{\gamma,\epsilon,w} \quad (3r_D r_T^3) \quad (10333)$$

$$\tau^{12}_{\gamma,\delta,w} = \sum_{\epsilon \in A} Z_{\epsilon,\gamma} \tau^{11}_{\epsilon,\delta,w} \quad (2r_D r_T^3) \quad (10334)$$

$${}^2R^3_{a,\gamma} \leftarrow - \sum_{\delta \in A} \sum_{w \in D} \frac{1}{2} {}^2D^3_{a,w} Y^3_{a,\delta} \tau^0_{\delta,\gamma,w} \tau^{12}_{\delta,\gamma,w} \quad (4r_D r_T^2 N_v) \quad (10335)$$

Raw expression

$${}^2R^3_{b,\zeta} \leftarrow - \sum_{\gamma \in A} \sum_{i \in O} \sum_{j \in O} \sum_{k \in O} \sum_{l \in O} \sum_{a \in V} \sum_{c \in V} \sum_{d \in V} \frac{1}{2} \quad (10336)$$

$$Y^{1,*}_{a,\gamma} Y^{2,*}_{i,\gamma} Z^*_{\gamma,\zeta} Y^{4,*}_{j,\zeta} {}^2D^{a,i,b,j} {}^2T_{c,k,b,j} {}^2T_{d,l,a,i} V_{l,c,k,d}$$

Factorized expression

$$\tau^0_{\gamma,\delta,w} = \sum_{i \in O} {}^2D^4_{i,w} Y^2_{i,\gamma} Y^{4,*}_{i,\delta} \quad (3r_D r_T^2 N_o) \quad (10337)$$

$$\tau^1_{\gamma,\delta,w} = \sum_{a \in V} {}^2D^1_{a,w} Y^3_{a,\gamma} Y^{1,*}_{a,\delta} \quad (3r_D r_T^2 N_v) \quad (10338)$$

$$\tau^2_{\gamma,\delta,w} = \sum_{i \in O} {}^2D^2_{i,w} Y^4_{i,\gamma} Y^{2,*}_{i,\delta} \quad (3r_D r_T^2 N_o) \quad (10339)$$

$$\tau^3_{\gamma,\delta,w} = \sum_{\epsilon \in A} Z^*_{\epsilon,\delta} \tau^1_{\gamma,\epsilon,w} \tau^2_{\gamma,\epsilon,w} \quad (3r_D r_T^3) \quad (10340)$$

$$\tau^4_{\gamma,\delta,w} = \sum_{\epsilon \in A} Z_{\gamma,\epsilon} \tau^3_{\epsilon,\delta,w} \quad (2r_D r_T^3) \quad (10341)$$

$$\tau^5_{\gamma,\alpha} = \sum_{a \in V} W^2_{a,\alpha} Y^1_{a,\gamma} \quad (2r_T r_V N_v) \quad (10342)$$

$$\tau^6_{\gamma,\alpha} = \sum_{i \in O} W^1_{i,\alpha} Y^2_{i,\gamma} \quad (2r_T r_V N_o) \quad (10343)$$

$$\tau^7_{\gamma,\alpha} = \sum_{\beta \in B} X_{\beta,\alpha} \tau^5_{\gamma,\beta} \tau^6_{\gamma,\beta} \quad (3r_T r_V^2) \quad (10344)$$

$$\tau^8_{\gamma,\alpha} = \sum_{\delta \in A} Z_{\delta,\gamma} \tau^7_{\delta,\alpha} \quad (2r_T^2 r_V) \quad (10345)$$

$$\tau^9_{\gamma,\alpha} = \sum_{i \in O} W^3_{i,\alpha} Y^4_{i,\gamma} \quad (2r_T r_V N_o) \quad (10346)$$

$$\tau^{10}_{\gamma,a} = \sum_{\alpha \in B} W^4_{a,\alpha} \tau^8_{\gamma,\alpha} \tau^9_{\gamma,\alpha} \quad (3r_T r_V N_v) \quad (10347)$$

$$\tau^{11}_{\gamma,\delta} = \sum_{a \in V} Y^1_{a,\gamma} \tau^{10}_{\delta,a} \quad (2r_T^2 N_v) \quad (10348)$$

$$\tau^{12}_{\gamma,a} = \sum_{\delta \in A} Y^3_{a,\delta} \tau^{11}_{\gamma,\delta} \quad (2r_T^2 N_v) \quad (10349)$$

$${}^2R^3_{a,\gamma} \leftarrow - \sum_{\delta \in A} \sum_{w \in D} \frac{1}{2} {}^2D^3_{a,w} \tau^{12}_{\delta,a} \tau^0_{\delta,\gamma,w} \tau^4_{\delta,\gamma,w} \quad (4r_D r_T^2 N_v^{11})_{\gamma,\delta,w} = \sum_{\epsilon \in A} \sum_{i \in O} {}^2D^4_{i,w} Y^{4,*}_{i,\delta} \tau^{10}_{\gamma,\epsilon,i} \tau^2_{\epsilon,\delta,w} \quad (4r_D r_T^3 N_o) \quad (10350) \quad (10363)$$

Raw expression

$${}^2R^3_{b,\zeta} \leftarrow - \sum_{\gamma \in A} \sum_{i \in O} \sum_{j \in O} \sum_{k \in O} \sum_{l \in O} \sum_{a \in V} \sum_{c \in V} \sum_{d \in V} \frac{1}{2} \quad (10351)$$

$$Y^{1,*}_{a,\gamma} \quad Y^{2,*}_{i,\gamma} \quad Z^*_{\gamma,\zeta} \quad Y^{4,*}_{j,\zeta}$$

$${}^2D^{a,i,b,j}_{c,k,b,l} \quad {}^2T_{c,k,b,l} \quad {}^2T_{d,j,a,i} \quad V_{k,c,l,d}$$

Factorized expression

$$\tau^0_{\gamma,\delta,w} = \sum_{a \in V} {}^2D^1_{a,w} Y^3_{a,\gamma} Y^{1,*}_{a,\delta} \quad (3r_D r_T^2 N_v) \quad (10352)$$

$$\tau^1_{\gamma,\delta,w} = \sum_{i \in O} {}^2D^2_{i,w} Y^4_{i,\gamma} Y^{2,*}_{i,\delta} \quad (3r_D r_T^2 N_o) \quad (10353)$$

$$\tau^2_{\gamma,\delta,w} = \sum_{\epsilon \in A} Z^*_{\epsilon,\delta} \tau^0_{\gamma,\epsilon,w} \tau^1_{\gamma,\epsilon,w} \quad (3r_D r_T^3) \quad (10354)$$

$$\tau^3_{\gamma,\alpha} = \sum_{a \in V} W^2_{a,\alpha} Y^1_{a,\gamma} \quad (2r_T r_V N_v) \quad (10355)$$

$$\tau^4_{\gamma,\alpha} = \sum_{i \in O} W^1_{i,\alpha} Y^2_{i,\gamma} \quad (2r_T r_V N_o) \quad (10356)$$

$$\tau^5_{\gamma,\alpha} = \sum_{\beta \in B} X_{\beta,\alpha} \tau^3_{\gamma,\beta} \tau^4_{\gamma,\beta} \quad (3r_T r_V^2) \quad (10357)$$

$$\tau^6_{\gamma,\alpha} = \sum_{\delta \in A} Z_{\delta,\gamma} \tau^5_{\delta,\alpha} \quad (2r_T^2 r_V) \quad (10358)$$

$$\tau^7_{\gamma,\alpha} = \sum_{a \in V} W^4_{a,\alpha} Y^1_{a,\gamma} \quad (2r_T r_V N_v) \quad (10359)$$

$$\tau^8_{\gamma,\delta,i} = \sum_{\alpha \in B} W^3_{i,\alpha} \tau^6_{\delta,\alpha} \tau^7_{\gamma,\alpha} \quad (3r_T^2 r_V N_o) \quad (10360)$$

$$\tau^9_{\gamma,\delta,\epsilon} = \sum_{i \in O} Z_{\gamma,\delta} Y^4_{i,\delta} \tau^8_{\gamma,\epsilon,i} \quad (3r_T^3 N_o) \quad (10361)$$

$$\tau^{10}_{\gamma,\delta,i} = \sum_{\epsilon \in A} Y^2_{i,\epsilon} \tau^9_{\epsilon,\gamma,\delta} \quad (2r_T^3 N_o) \quad (10362)$$

$${}^2R^3_{a,\gamma} \leftarrow - \sum_{\delta \in A} \sum_{w \in D} \frac{1}{2} {}^2D^3_{a,w} Y^3_{a,\delta} \tau^{11}_{\delta,\gamma,w} \quad (3r_D r_T^2 N_v) \quad (10364)$$

Raw expression

$${}^2R^3_{b,\zeta} \leftarrow \sum_{\gamma \in A} \sum_{i \in O} \sum_{j \in O} \sum_{k \in O} \sum_{l \in O} \sum_{a \in V} \sum_{c \in V} \sum_{d \in V} \frac{1}{4} \quad (10365)$$

$$Y^{1,*}_{a,\gamma} \quad Y^{2,*}_{i,\gamma} \quad Z^*_{\gamma,\zeta} \quad Y^{4,*}_{j,\zeta}$$

$${}^2D^{a,i,b,j}_{c,k,b,l} \quad {}^2T_{a,i,b,k} \quad {}^2T_{c,j,d,l} \quad V_{k,d,l,c}$$

Factorized expression

$$\tau^0_{\gamma,\delta,w} = \sum_{a \in V} {}^2D^1_{a,w} Y^1_{a,\gamma} Y^{1,*}_{a,\delta} \quad (3r_D r_T^2 N_v) \quad (10366)$$

$$\tau^1_{\gamma,\delta,w} = \sum_{i \in O} {}^2D^2_{i,w} Y^2_{i,\gamma} Y^{2,*}_{i,\delta} \quad (3r_D r_T^2 N_o) \quad (10367)$$

$$\tau^2_{\gamma,\delta,w} = \sum_{\epsilon \in A} Z^*_{\epsilon,\delta} \tau^0_{\gamma,\epsilon,w} \tau^1_{\gamma,\epsilon,w} \quad (3r_D r_T^3) \quad (10368)$$

$$\tau^3_{\gamma,\delta,w} = \sum_{\epsilon \in A} Z_{\epsilon,\gamma} \tau^2_{\epsilon,\delta,w} \quad (2r_D r_T^3) \quad (10369)$$

$$\tau^4_{\gamma,\alpha} = \sum_{a \in V} W^2_{a,\alpha} Y^1_{a,\gamma} \quad (2r_T r_V N_v) \quad (10370)$$

$$\tau^5_{\gamma,\alpha,i} = \sum_{\beta \in B} W^1_{i,\beta} X_{\beta,\alpha} \tau^4_{\gamma,\beta} \quad (3r_T r_V^2 N_o) \quad (10371)$$

$$\tau^6_{\gamma,\alpha} = \sum_{i \in O} W^3_{i,\alpha} Y^2_{i,\gamma} \quad (2r_T r_V N_o) \quad (10372)$$

$$\tau^7_{\gamma,\alpha} = \sum_{a \in V} W^4_{a,\alpha} Y^3_{a,\gamma} \quad (2r_T r_V N_v) \quad (10373)$$

$$\tau^8_{\gamma,\delta,i} = \sum_{\alpha \in B} \tau^6_{\gamma,\alpha} \tau^7_{\delta,\alpha} \tau^5_{\gamma,\alpha,i} \quad (3r_T^2 r_V N_o) \quad (10374)$$

$$\tau^9_{\gamma,i} = \sum_{\delta \in A} Z_{\delta,\gamma} \tau^8_{\delta,\gamma,i} \quad (2r_T^2 N_o) \quad (10375)$$

$$\tau^{10}_{i,j} = \sum_{\gamma \in A} Y^4_{j,\gamma} \tau^9_{\gamma,i} \quad (2r_T N_o^2) \quad (10376)$$

$$\tau^7_{i,j,k,l} = \sum_{\gamma \in A} Y^2_{k,\gamma} \tau^6_{\gamma,i,j,l} \quad (2r_T N_o^4) \quad (10388)$$

$$\tau^{11}_{\gamma,i} = \sum_{j \in O} Y^4_{j,\gamma} \tau^{10}_{j,i} \quad (2r_T N_o^2) \quad (10377)$$

$$\tau^8_{\gamma,i,j,k} = \sum_{l \in O} Y^2_{l,\gamma} \tau^7_{l,i,j,k} \quad (2r_T N_o^4) \quad (10389)$$

$$\tau^{12}_{\gamma,\delta,w} = \sum_{i \in O} {}^2D^4_{i,w} Y^{4,*}_{i,\delta} \tau^{11}_{\gamma,i} \quad (3r_D r_T^2 N_o) \quad (10378)$$

$$\tau^9_{\gamma,\delta,w,i} = \sum_{j \in O} \sum_{k \in O} {}^2D^2_{j,w} {}^2D^4_{k,w} Y^{4,*}_{k,\delta} \tau^1_{\gamma,\delta,w,j} \tau^8_{\gamma,i,j,k} \quad (5r_D r_T^2 N_o) \quad (10390)$$

$${}^2R^3_{a,\gamma} \leftarrow \sum_{\delta \in A} \sum_{w \in D} \frac{1}{4} {}^2D^3_{a,w} Y^3_{a,\delta} \tau^{12}_{\delta,\gamma,w} \tau^3_{\delta,\gamma,w} \quad (4r_D r_T^2 N_v) \quad (10379)$$

$$\tau^{10}_{\gamma,\delta,w} = \sum_{\epsilon \in A} \sum_{i \in O} Z_{\epsilon,\gamma} Y^4_{i,\gamma} \tau^9_{\epsilon,\delta,w,i} \quad (3r_D r_T^3 N_o) \quad (10391)$$

Raw expression

$${}^2R^3_{b,\zeta} \leftarrow \sum_{\gamma \in A} \sum_{i \in O} \sum_{j \in O} \sum_{k \in O} \sum_{l \in O} \sum_{a \in V} \sum_{c \in V} \sum_{d \in V} \frac{1}{4} \quad (10380)$$

$$Y^{1,*}_{a,\gamma} \quad Y^{2,*}_{i,\gamma} \quad Z^*_{\gamma,\zeta} \quad Y^{4,*}_{j,\zeta}$$

$${}^2D^{a,i,b,j} \quad {}^2T_{a,i,b,k} \quad {}^2T_{c,l,d,j} \quad V_{k,c,l,d}$$

$${}^2R^3_{a,\gamma} \leftarrow \sum_{\delta \in A} \sum_{w \in D} \frac{1}{4} {}^2D^3_{a,w} Y^3_{a,\delta} \tau^{10}_{\delta,\gamma,w} \quad (3r_D r_T^2 N_v) \quad (10392)$$

Raw expression

Factorized expression

$$\tau^0_{\gamma,\delta,w} = \sum_{a \in V} {}^2D^1_{a,w} Y^1_{a,\gamma} Y^{1,*}_{a,\delta} \quad (3r_D r_T^2 N_v) \quad (10381)$$

$${}^2R^3_{b,\zeta} \leftarrow \sum_{\gamma \in A} \sum_{i \in O} \sum_{j \in O} \sum_{k \in O} \sum_{l \in O} \sum_{a \in V} \sum_{c \in V} \sum_{d \in V} \frac{1}{4} \quad (10393)$$

$$Y^{1,*}_{a,\gamma} \quad Y^{2,*}_{i,\gamma} \quad Z^*_{\gamma,\zeta} \quad Y^{4,*}_{j,\zeta}$$

$${}^2D^{a,i,b,j} \quad {}^2T_{a,i,d,j} \quad {}^2T_{b,k,c,l} \quad V_{k,c,l,d}$$

Factorized expression

$$\tau^1_{\gamma,\delta,w,i} = \sum_{\epsilon \in A} Y^{2,*}_{i,\epsilon} Z^*_{\epsilon,\delta} \tau^0_{\gamma,\epsilon,w} \quad (3r_D r_T^3 N_o) \quad (10382)$$

$$\tau^0_{\gamma,\delta,w} = \sum_{i \in O} {}^2D^4_{i,w} Y^4_{i,\gamma} Y^{4,*}_{i,\delta} \quad (3r_D r_T^2 N_o) \quad (10394)$$

$$\tau^2_{\gamma,\alpha} = \sum_{a \in V} W^2_{a,\alpha} Y^1_{a,\gamma} \quad (2r_T r_V N_v) \quad (10383)$$

$$\tau^1_{\gamma,\alpha} = \sum_{a \in V} W^2_{a,\alpha} Y^1_{a,\gamma} \quad (2r_T r_V N_v) \quad (10395)$$

$$\tau^3_{\gamma,\alpha,i} = \sum_{\beta \in B} W^1_{i,\beta} X_{\beta,\alpha} \tau^2_{\gamma,\beta} \quad (3r_T r_V^2 N_o) \quad (10384)$$

$$\tau^2_{\gamma,\alpha,i} = \sum_{\beta \in B} W^1_{i,\beta} X_{\beta,\alpha} \tau^1_{\gamma,\beta} \quad (3r_T r_V^2 N_o) \quad (10396)$$

$$\tau^4_{\gamma,\alpha} = \sum_{a \in V} W^4_{a,\alpha} Y^3_{a,\gamma} \quad (2r_T r_V N_v) \quad (10385)$$

$$\tau^3_{\gamma,\alpha} = \sum_{i \in O} W^3_{i,\alpha} Y^2_{i,\gamma} \quad (2r_T r_V N_o) \quad (10397)$$

$$\tau^5_{\gamma,\alpha,i} = \sum_{\delta \in A} Z_{\gamma,\delta} Y^4_{i,\delta} \tau^4_{\delta,\alpha} \quad (3r_T^2 r_V N_o) \quad (10386)$$

$$\tau^4_{\gamma,\alpha} = \sum_{a \in V} W^4_{a,\alpha} Y^3_{a,\gamma} \quad (2r_T r_V N_v) \quad (10398)$$

$$\tau^6_{\gamma,i,j,k} = \sum_{\alpha \in B} W^3_{j,\alpha} \tau^3_{\gamma,\alpha,i} \tau^5_{\gamma,\alpha,k} \quad (3r_T r_V N_o^3) \quad (10387)$$

$$\tau^5_{\gamma,\delta,i} = \sum_{\alpha \in B} \tau^3_{\gamma,\alpha} \tau^4_{\delta,\alpha} \tau^2_{\gamma,\alpha,i} \quad (3r_T^2 r_V N_o) \quad (10399)$$



$$\tau^6_{\gamma,i} = \sum_{\delta \in A} Z_{\delta,\gamma} \tau^5_{\delta,\gamma,i} \quad (2r_T^2 N_o) \quad (10400)$$

$$\tau^4_{\gamma,\alpha} = \sum_{a \in V} W^2_{a,\alpha} Y^3_{a,\gamma} \quad (2r_T r_V N_v) \quad (10413)$$

$$\tau^7_{i,j} = \sum_{\gamma \in A} Y^4_{j,\gamma} \tau^6_{\gamma,i} \quad (2r_T N_o^2) \quad (10401)$$

$$\tau^5_{\gamma,\alpha,i} = \sum_{\beta \in B} W^1_{i,\beta} X_{\beta,\alpha} \tau^4_{\gamma,\beta} \quad (3r_T r_V^2 N_o) \quad (10414)$$

$$\tau^8_{\gamma,i} = \sum_{j \in O} Y^2_{j,\gamma} \tau^7_{j,i} \quad (2r_T N_o^2) \quad (10402)$$

$$\tau^6_{\gamma,\alpha} = \sum_{i \in O} W^3_{i,\alpha} Y^4_{i,\gamma} \quad (2r_T r_V N_o) \quad (10415)$$

$$\tau^9_{\gamma,\delta,w} = \sum_{i \in O} {}^2D^2_{i,w} Y^{2,*}_{i,\delta} \tau^8_{\gamma,i} \quad (3r_D r_T^2 N_o) \quad (10403)$$

$$\tau^7_{\gamma,\alpha} = \sum_{a \in V} W^4_{a,\alpha} Y^1_{a,\gamma} \quad (2r_T r_V N_v) \quad (10416)$$

$$\tau^{10}_{\gamma,\delta,w} = \sum_{a \in V} {}^2D^1_{a,w} Y^1_{a,\gamma} Y^{1,*}_{a,\delta} \quad (3r_D r_T^2 N_v) \quad (10404)$$

$$\tau^8_{\gamma,\delta,i} = \sum_{\alpha \in B} \tau^6_{\delta,\alpha} \tau^7_{\gamma,\alpha} \tau^5_{\delta,\alpha,i} \quad (3r_T^2 r_V N_o) \quad (10417)$$

$$\tau^{11}_{\gamma,\delta,w} = \sum_{\epsilon \in A} Z^*_{\epsilon,\delta} \tau^{10}_{\gamma,\epsilon,w} \tau^9_{\gamma,\epsilon,w} \quad (3r_D r_T^3) \quad (10405)$$

$$\tau^9_{\gamma,i} = \sum_{\delta \in A} Z_{\gamma,\delta} \tau^8_{\gamma,\delta,i} \quad (2r_T^2 N_o) \quad (10418)$$

$$\tau^{12}_{\gamma,\delta,w} = \sum_{\epsilon \in A} Z_{\epsilon,\gamma} \tau^{11}_{\epsilon,\delta,w} \quad (2r_D r_T^3) \quad (10406)$$

$$\tau^{10}_{i,j} = \sum_{\gamma \in A} Y^2_{j,\gamma} \tau^9_{\gamma,i} \quad (2r_T N_o^2) \quad (10419)$$

$${}^2R^3_{a,\gamma} \leftarrow \sum_{\delta \in A} \sum_{w \in D} \frac{1}{4} {}^2D^3_{a,w} Y^3_{a,\delta} \tau^0_{\delta,\gamma,w} \tau^{12}_{\delta,\gamma,w} \quad (4r_D r_T^2 N_v) \quad (10407)$$

$$\tau^{11}_{\gamma,i} = \sum_{j \in O} Y^4_{j,\gamma} \tau^{10}_{j,i} \quad (2r_T N_o^2) \quad (10420)$$

Raw expression

$$\tau^{12}_{\gamma,\delta,w} = \sum_{i \in O} {}^2D^4_{i,w} Y^{4,*}_{i,\delta} \tau^{11}_{\gamma,i} \quad (3r_D r_T^2 N_o) \quad (10421)$$

$${}^2R^3_{b,\zeta} \leftarrow \sum_{\gamma \in A} \sum_{i \in O} \sum_{j \in O} \sum_{k \in O} \sum_{l \in O} \sum_{a \in V} \sum_{c \in V} \sum_{d \in V} \frac{1}{4} \quad (10408)$$

$$Y^{1,*}_{a,\gamma} \quad Y^{2,*}_{i,\gamma} \quad Z^*_{\gamma,\zeta} \quad Y^{4,*}_{j,\zeta}$$

$${}^2D^{a,i,b,j} \quad {}^2T_{a,i,d,j} \quad {}^2T_{c,k,b,l} \quad V_{k,d,l,c}$$

$${}^2R^3_{a,\gamma} \leftarrow \sum_{\delta \in A} \sum_{w \in D} \frac{1}{4} {}^2D^3_{a,w} Y^3_{a,\delta} \tau^{12}_{\delta,\gamma,w} \tau^3_{\delta,\gamma,w} \quad (4r_D r_T^2 N_v) \quad (10422)$$

Factorized expression

Raw expression

$$\tau^0_{\gamma,\delta,w} = \sum_{a \in V} {}^2D^1_{a,w} Y^1_{a,\gamma} Y^{1,*}_{a,\delta} \quad (3r_D r_T^2 N_v) \quad (10409)$$

$${}^2R^3_{b,\zeta} \leftarrow \sum_{\gamma \in A} \sum_{i \in O} \sum_{j \in O} \sum_{k \in O} \sum_{l \in O} \sum_{a \in V} \sum_{c \in V} \sum_{d \in V} \frac{1}{4} \quad (10423)$$

$$Y^{1,*}_{a,\gamma} \quad Y^{2,*}_{i,\gamma} \quad Z^*_{\gamma,\zeta} \quad Y^{4,*}_{j,\zeta}$$

$${}^2D^{a,i,b,j} \quad {}^2T_{a,i,d,l} \quad {}^2T_{b,k,c,j} \quad V_{l,c,k,d}$$

$$\tau^1_{\gamma,\delta,w} = \sum_{i \in O} {}^2D^2_{i,w} Y^2_{i,\gamma} Y^{2,*}_{i,\delta} \quad (3r_D r_T^2 N_o) \quad (10410)$$

Factorized expression

$$\tau^2_{\gamma,\delta,w} = \sum_{\epsilon \in A} Z^*_{\epsilon,\delta} \tau^0_{\gamma,\epsilon,w} \tau^1_{\gamma,\epsilon,w} \quad (3r_D r_T^3) \quad (10411)$$

$$\tau^0_{\gamma,\delta,w} = \sum_{i \in O} {}^2D^4_{i,w} Y^4_{i,\gamma} Y^{4,*}_{i,\delta} \quad (3r_D r_T^2 N_o) \quad (10424)$$

$$\tau^3_{\gamma,\delta,w} = \sum_{\epsilon \in A} Z_{\epsilon,\gamma} \tau^2_{\epsilon,\delta,w} \quad (2r_D r_T^3) \quad (10412)$$

$$\tau^1_{\gamma,\alpha} = \sum_{a \in V} W^2_{a,\alpha} Y^3_{a,\gamma} \quad (2r_T r_V N_v) \quad (10425)$$

$$\tau^2_{\gamma,\alpha,i} = \sum_{\beta \in B} W^1_{i,\beta} X_{\beta,\alpha} \tau^1_{\gamma,\beta} \quad (3r_T r_V^2 N_o) \quad (10426)$$

$$\tau^3_{\gamma,\alpha} = \sum_{i \in O} W^3_{i,\alpha} Y^4_{i,\gamma} \quad (2r_T r_V N_o) \quad (10427)$$

$$\tau^4_{\gamma,\alpha} = \sum_{a \in V} W^4_{a,\alpha} Y^1_{a,\gamma} \quad (2r_T r_V N_v) \quad (10428)$$

$$\tau^5_{\gamma,\delta,i} = \sum_{\alpha \in B} \tau^3_{\delta,\alpha} \tau^4_{\gamma,\alpha} \tau^2_{\delta,\alpha,i} \quad (3r_T^2 r_V N_o) \quad (10429)$$

$$\tau^6_{\gamma,i} = \sum_{\delta \in A} Z_{\gamma,\delta} \tau^5_{\gamma,\delta,i} \quad (2r_T^2 N_o) \quad (10430)$$

$$\tau^7_{i,j} = \sum_{\gamma \in A} Y^2_{j,\gamma} \tau^6_{\gamma,i} \quad (2r_T N_o^2) \quad (10431)$$

$$\tau^8_{\gamma,i} = \sum_{j \in O} Y^2_{j,\gamma} \tau^7_{j,i} \quad (2r_T N_o^2) \quad (10432)$$

$$\tau^9_{\gamma,\delta,w} = \sum_{i \in O} {}^2D^2_{i,w} Y^{2,*}_{i,\delta} \tau^8_{\gamma,i} \quad (3r_D r_T^2 N_o) \quad (10433)$$

$$\tau^{10}_{\gamma,\delta,w} = \sum_{a \in V} {}^2D^1_{a,w} Y^1_{a,\gamma} Y^{1,*}_{a,\delta} \quad (3r_D r_T^2 N_v) \quad (10434)$$

$$\tau^{11}_{\gamma,\delta,w} = \sum_{\epsilon \in A} Z^*_{\epsilon,\delta} \tau^{10}_{\gamma,\epsilon,w} \tau^9_{\gamma,\epsilon,w} \quad (3r_D r_T^3) \quad (10435)$$

$$\tau^{12}_{\gamma,\delta,w} = \sum_{\epsilon \in A} Z_{\epsilon,\gamma} \tau^{11}_{\epsilon,\delta,w} \quad (2r_D r_T^3) \quad (10436)$$

$${}^2R^3_{a,\gamma} \leftarrow \sum_{\delta \in A} \sum_{w \in D} \frac{1}{4} {}^2D^3_{a,w} Y^3_{a,\delta} \tau^0_{\delta,\gamma,w} \tau^{12}_{\delta,\gamma,w} \quad (4r_D r_T^2 N_v) \quad (10437)$$

Raw expression

$${}^2R^3_{b,\zeta} \leftarrow \sum_{\gamma \in A} \sum_{i \in O} \sum_{j \in O} \sum_{k \in O} \sum_{l \in O} \sum_{a \in V} \sum_{c \in V} \sum_{d \in V} \frac{1}{4} \quad (10438)$$

$$Y^{1,*}_{a,\gamma} Y^{2,*}_{i,\gamma} Z^*_{\gamma,\zeta} Y^{4,*}_{j,\zeta} {}^2D^{a,i,b,j} {}^2T_{a,i,d,l} {}^2T_{c,j,b,k} V_{l,c,k,d}$$

Factorized expression

$$\tau^0_{\gamma,\delta,w} = \sum_{a \in V} {}^2D^1_{a,w} Y^1_{a,\gamma} Y^{1,*}_{a,\delta} \quad (3r_D r_T^2 N_v) \quad (10439)$$

$$\tau^1_{\gamma,\delta,w,i} = \sum_{\epsilon \in A} Y^{2,*}_{i,\epsilon} Z^*_{\epsilon,\delta} \tau^0_{\gamma,\epsilon,w} \quad (3r_D r_T^3 N_o) \quad (10440)$$

$$\tau^2_{\gamma,\alpha} = \sum_{a \in V} W^4_{a,\alpha} Y^1_{a,\gamma} \quad (2r_T r_V N_v) \quad (10441)$$

$$\tau^3_{\gamma,\alpha,i} = \sum_{\beta \in B} X_{\alpha,\beta} W^3_{i,\beta} \tau^2_{\gamma,\beta} \quad (3r_T r_V^2 N_o) \quad (10442)$$

$$\tau^4_{\gamma,\alpha} = \sum_{a \in V} W^2_{a,\alpha} Y^3_{a,\gamma} \quad (2r_T r_V N_v) \quad (10443)$$

$$\tau^5_{\gamma,\alpha,i} = \sum_{\delta \in A} Z_{\gamma,\delta} Y^4_{i,\delta} \tau^4_{\delta,\alpha} \quad (3r_T^2 r_V N_o) \quad (10444)$$

$$\tau^6_{\gamma,i,j,k} = \sum_{\alpha \in B} W^1_{i,\alpha} \tau^3_{\gamma,\alpha,j} \tau^5_{\gamma,\alpha,k} \quad (3r_T r_V N_o^3) \quad (10445)$$

$$\tau^7_{i,j,k,l} = \sum_{\gamma \in A} Y^2_{k,\gamma} \tau^6_{\gamma,i,j,l} \quad (2r_T N_o^4) \quad (10446)$$

$$\tau^8_{\gamma,i,j,k} = \sum_{l \in O} Y^2_{l,\gamma} \tau^7_{l,i,j,k} \quad (2r_T N_o^4) \quad (10447)$$

$$\tau^9_{\gamma,\delta,w,i} = \sum_{j \in O} \sum_{k \in O} {}^2D^2_{j,w} {}^2D^4_{k,w} Y^{4,*}_{k,\delta} \tau^1_{\gamma,\delta,w,j} \tau^8_{\gamma,i,k,j} \quad (5r_D r_T^2 N_o) \quad (10448)$$

$$\tau^{10}_{\gamma,\delta,w} = \sum_{\epsilon \in A} \sum_{i \in O} Z_{\epsilon,\gamma} Y^4_{i,\gamma} \tau^9_{\epsilon,\delta,w,i} \quad (3r_D r_T^3 N_o) \quad (10449)$$

$${}^2R^3_{a,\gamma} \leftarrow \sum_{\delta \in A} \sum_{w \in D} \frac{1}{4} {}^2D^3_{a,w} Y^3_{a,\delta} \tau^{10}_{\delta,\gamma,w} \quad (3r_D r_T^2 N_v) \quad (10450)$$

Raw expression

$${}^2R^3_{b,\zeta} \leftarrow \sum_{\gamma \in A} \sum_{i \in O} \sum_{j \in O} \sum_{k \in O} \sum_{l \in O} \sum_{a \in V} \sum_{c \in V} \sum_{d \in V} \frac{1}{4} \quad (10451)$$

$$Y^{1,*}_{a,\gamma} Y^{2,*}_{i,\gamma} Z^*_{\gamma,\zeta} Y^{4,*}_{j,\zeta} {}^2D^{a,i,b,j} {}^2T_{a,k,b,j} {}^2T_{c,i,d,l} V_{k,d,l,c}$$

Factorized expression

$$\tau^0_{\gamma,\delta,w} = \sum_{i \in O} {}^2D^4_{i,w} Y^4_{i,\gamma} Y^{4,*}_{i,\delta} \quad (3r_D r_T^2 N_o) \quad (10452)$$

$$\tau^1_{\gamma,\delta,w} = \sum_{a \in V} {}^2D^1_{a,w} Y^1_{a,\gamma} Y^{1,*}_{a,\delta} \quad (3r_D r_T^2 N_v) \quad (10453)$$

$$\tau^2_{\gamma,\delta,w} = \sum_{i \in O} {}^2D^2_{i,w} Y^2_{i,\gamma} Y^{2,*}_{i,\delta} \quad (3r_D r_T^2 N_o) \quad (10454)$$

$$\tau^3_{\gamma,\delta,w} = \sum_{\epsilon \in A} Z^*_{\epsilon,\delta} \tau^1_{\gamma,\epsilon,w} \tau^2_{\gamma,\epsilon,w} \quad (3r_D r_T^3) \quad (10455)$$

$$\tau^4_{\gamma,\delta,w} = \sum_{\epsilon \in A} Z_{\epsilon,\gamma} \tau^3_{\epsilon,\delta,w} \quad (2r_D r_T^3) \quad (10456)$$

$$\tau^5_{\gamma,\alpha} = \sum_{a \in V} W^2_{a,\alpha} Y^3_{a,\gamma} \quad (2r_T r_V N_v) \quad (10457)$$

$$\tau^6_{\gamma,\alpha,i} = \sum_{\beta \in B} W^1_{i,\beta} X_{\beta,\alpha} \tau^5_{\gamma,\beta} \quad (3r_T r_V^2 N_o) \quad (10458)$$

$$\tau^7_{\gamma,\alpha} = \sum_{i \in O} W^3_{i,\alpha} Y^4_{i,\gamma} \quad (2r_T r_V N_o) \quad (10459)$$

$$\tau^8_{\gamma,\alpha} = \sum_{\delta \in A} \sum_{i \in O} Y^2_{i,\gamma} Z_{\gamma,\delta} \tau^7_{\delta,\alpha} \tau^6_{\delta,\alpha,i} \quad (4r_T^2 r_V N_o) \quad (10460)$$

$$\tau^9_{\gamma,a} = \sum_{\alpha \in B} W^4_{a,\alpha} \tau^8_{\gamma,\alpha} \quad (2r_T r_V N_v) \quad (10461)$$

$$\tau^{10}_{\gamma,\delta} = \sum_{a \in V} Y^3_{a,\delta} \tau^9_{\gamma,a} \quad (2r_T^2 N_v) \quad (10462)$$

$$\tau^{11}_{\gamma,a} = \sum_{\delta \in A} Y^1_{a,\delta} \tau^{10}_{\delta,\gamma} \quad (2r_T^2 N_v) \quad (10463)$$

$${}^2R^3_{a,\gamma} \leftarrow \sum_{\delta \in A} \sum_{w \in D} \frac{1}{4} {}^2D^3_{a,w} \tau^{11}_{\delta,a} \tau^0_{\delta,\gamma,w} \tau^4_{\delta,\gamma,w} \quad (4r_D r_T^2 N_v) \quad (10464)$$

Raw expression

$${}^2R^3_{b,\zeta} \leftarrow \sum_{\gamma \in A} \sum_{i \in O} \sum_{j \in O} \sum_{k \in O} \sum_{l \in O} \sum_{a \in V} \sum_{c \in V} \sum_{d \in V} \frac{1}{4} \quad (10465)$$

$$Y^{1,*}_{a,\gamma} Y^{2,*}_{i,\gamma} Z^*_{\gamma,\zeta} Y^{4,*}_{j,\zeta}$$

$${}^2D^{a,i,b,j} {}^2T_{a,k,b,j} {}^2T_{c,l,d,i} V_{k,c,l,d}$$

Factorized expression

$$\tau^0_{\gamma,\delta,w} = \sum_{a \in V} {}^2D^1_{a,w} Y^1_{a,\gamma} Y^{1,*}_{a,\delta} \quad (3r_D r_T^2 N_v) \quad (10466)$$

$$\tau^1_{\gamma,\delta,w} = \sum_{i \in O} {}^2D^2_{i,w} Y^2_{i,\gamma} Y^{2,*}_{i,\delta} \quad (3r_D r_T^2 N_o) \quad (10467)$$

$$\tau^2_{\gamma,\delta,w} = \sum_{\epsilon \in A} Z^*_{\epsilon,\delta} \tau^0_{\gamma,\epsilon,w} \tau^1_{\gamma,\epsilon,w} \quad (3r_D r_T^3) \quad (10468)$$

$$\tau^3_{\gamma,\delta,w} = \sum_{\epsilon \in A} Z_{\epsilon,\gamma} \tau^2_{\epsilon,\delta,w} \quad (2r_D r_T^3) \quad (10469)$$

$$\tau^4_{\gamma,\alpha} = \sum_{a \in V} W^4_{a,\alpha} Y^3_{a,\gamma} \quad (2r_T r_V N_v) \quad (10470)$$

$$\tau^5_{\gamma,\alpha,i} = \sum_{\beta \in B} X_{\alpha,\beta} W^3_{i,\beta} \tau^4_{\gamma,\beta} \quad (3r_T r_V^2 N_o) \quad (10471)$$

$$\tau^6_{\gamma,\alpha} = \sum_{i \in O} W^1_{i,\alpha} Y^4_{i,\gamma} \quad (2r_T r_V N_o) \quad (10472)$$

$$\tau^7_{\gamma,\alpha} = \sum_{a \in V} W^2_{a,\alpha} Y^3_{a,\gamma} \quad (2r_T r_V N_v) \quad (10473)$$

$$\tau^8_{\gamma,\delta,i} = \sum_{\alpha \in B} \tau^6_{\gamma,\alpha} \tau^7_{\delta,\alpha} \tau^5_{\gamma,\alpha,i} \quad (3r_T^2 r_V N_o) \quad (10474)$$

$$\tau^9_{\gamma,\delta,\epsilon} = \sum_{i \in O} Y^2_{i,\gamma} Z_{\gamma,\delta} \tau^8_{\epsilon,\delta,i} \quad (3r_T^3 N_o) \quad (10475)$$

$$\tau^{10}_{\gamma,\delta,i} = \sum_{\epsilon \in A} Y^4_{i,\epsilon} \tau^9_{\gamma,\epsilon,\delta} \quad (2r_T^3 N_o) \quad (10476)$$

$$\tau^{11}_{\gamma,\delta,w} = \sum_{\epsilon \in A} \sum_{i \in O} {}^2D^4_{i,w} Y^{4,*}_{i,\delta} \tau^{10}_{\gamma,\epsilon,i} \tau^3_{\epsilon,\delta,w} \quad (4r_D r_T^3 N_o) \quad (10477)$$

$${}^2R^3_{a,\gamma} \leftarrow \sum_{\delta \in A} \sum_{w \in D} \frac{1}{4} {}^2D^3_{a,w} Y^1_{a,\delta} \tau^{11}_{\delta,\gamma,w} \quad (3r_D r_T^2 N_v) \quad (10478)$$

Raw expression

$${}^2R^3_{b,\zeta} \leftarrow \sum_{\gamma \in A} \sum_{i \in O} \sum_{j \in O} \sum_{k \in O} \sum_{l \in O} \sum_{a \in V} \sum_{c \in V} \sum_{d \in V} \frac{1}{4} Y^{1,*}_{a,\gamma} Y^{2,*}_{i,\gamma} Z^*_{\gamma,\zeta} Y^{4,*}_{j,\zeta} {}^2D^{a,i,b,j} {}^2T_{a,k,b,l} {}^2T_{c,i,d,j} V_{k,c,l,d} \quad (10479)$$

Factorized expression

$$\tau^0_{\gamma,\delta,w} = \sum_{i \in O} {}^2D^4_{i,w} Y^2_{i,\gamma} Y^{4,*}_{i,\delta} \quad (3r_D r_T^2 N_o) \quad (10480)$$

$$\tau^1_{\gamma,\alpha} = \sum_{a \in V} W^2_{a,\alpha} Y^3_{a,\gamma} \quad (2r_T r_V N_v) \quad (10481)$$

$$\tau^2_{\gamma,\alpha,i} = \sum_{\beta \in B} W^1_{i,\beta} X_{\beta,\alpha} \tau^1_{\gamma,\beta} \quad (3r_T r_V^2 N_o) \quad (10482)$$

$$\tau^3_{\gamma,\alpha} = \sum_{i \in O} W^3_{i,\alpha} Y^4_{i,\gamma} \quad (2r_T r_V N_o) \quad (10483)$$

$$\tau^4_{\gamma,\alpha} = \sum_{\delta \in A} \sum_{i \in O} Y^2_{i,\gamma} Z_{\gamma,\delta} \tau^3_{\delta,\alpha} \tau^2_{\delta,\alpha,i} \quad (4r_T^2 r_V N_o) \quad (10484)$$

$$\tau^5_{\gamma,a} = \sum_{\alpha \in B} W^4_{a,\alpha} \tau^4_{\gamma,\alpha} \quad (2r_T r_V N_v) \quad (10485)$$

$$\tau^6_{\gamma,\delta} = \sum_{a \in V} Y^3_{a,\delta} \tau^5_{\gamma,a} \quad (2r_T^2 N_v) \quad (10486)$$

$$\tau^7_{\gamma,a} = \sum_{\delta \in A} Y^1_{a,\delta} \tau^6_{\delta,\gamma} \quad (2r_T^2 N_v) \quad (10487)$$

$$\tau^8_{\gamma,\delta,w} = \sum_{a \in V} {}^2D^1_{a,w} Y^{1,*}_{a,\delta} \tau^7_{\gamma,a} \quad (3r_D r_T^2 N_v) \quad (10488)$$

$$\tau^9_{\gamma,\delta,w} = \sum_{i \in O} {}^2D^2_{i,w} Y^4_{i,\gamma} Y^{2,*}_{i,\delta} \quad (3r_D r_T^2 N_o) \quad (10489)$$

$$\tau^{10}_{\gamma,\delta,w} = \sum_{\epsilon \in A} Z^*_{\epsilon,\delta} \tau^8_{\gamma,\epsilon,w} \tau^9_{\gamma,\epsilon,w} \quad (3r_D r_T^3) \quad (10490)$$

$$\tau^{11}_{\gamma,\delta,w} = \sum_{\epsilon \in A} Z_{\gamma,\epsilon} \tau^{10}_{\epsilon,\delta,w} \quad (2r_D r_T^3) \quad (10491)$$

$${}^2R^3_{a,\gamma} \leftarrow \sum_{\delta \in A} \sum_{w \in D} \frac{1}{4} {}^2D^3_{a,w} Y^1_{a,\delta} \tau^0_{\delta,\gamma,w} \tau^{11}_{\delta,\gamma,w} \quad (4r_D r_T^2 N_v) \quad (10492)$$

Raw expression

$${}^2R^3_{b,\zeta} \leftarrow \sum_{\gamma \in A} \sum_{i \in O} \sum_{j \in O} \sum_{k \in O} \sum_{l \in O} \sum_{a \in V} \sum_{c \in V} \sum_{d \in V} \frac{1}{4} Y^{1,*}_{a,\gamma} Y^{2,*}_{i,\gamma} Z^*_{\gamma,\zeta} Y^{4,*}_{j,\zeta} {}^2D^{a,i,b,j} {}^2T_{a,k,b,l} {}^2T_{c,j,d,i} V_{k,d,l,c} \quad (10493)$$

Factorized expression

$$\tau^0_{\gamma,\delta,w} = \sum_{a \in V} {}^2D^1_{a,w} Y^1_{a,\gamma} Y^{1,*}_{a,\delta} \quad (3r_D r_T^2 N_v) \quad (10494)$$

$$\tau^1_{\gamma,\alpha} = \sum_{a \in V} W^2_{a,\alpha} Y^3_{a,\gamma} \quad (2r_T r_V N_v) \quad (10495)$$

$$\tau^2_{\gamma,\alpha,i} = \sum_{\beta \in B} W^1_{i,\beta} X_{\beta,\alpha} \tau^1_{\gamma,\beta} \quad (3r_T r_V^2 N_o) \quad (10496)$$

$$\tau^3_{\gamma,\alpha} = \sum_{i \in O} W^3_{i,\alpha} Y^4_{i,\gamma} \quad (2r_T r_V N_o) \quad (10497)$$

$$\tau^4_{\gamma,\alpha} = \sum_{a \in V} W^4_{a,\alpha} Y^3_{a,\gamma} \quad (2r_T r_V N_v) \quad (10498)$$

$$\tau^5_{\gamma,\delta,i} = \sum_{\alpha \in B} \tau^3_{\gamma,\alpha} \tau^4_{\delta,\alpha} \tau^2_{\gamma,\alpha,i} \quad (3r_T^2 r_V N_o) \quad (10499)$$

$$\tau^6_{\gamma,\delta,\epsilon} = \sum_{i \in O} Y^2_{i,\gamma} Z_{\gamma,\delta} \tau^5_{\epsilon,\delta,i} \quad (3r_T^3 N_o) \quad (10500)$$

$$\tau^7_{\gamma,\delta,i} = \sum_{\epsilon \in A} Y^4_{i,\epsilon} \tau^6_{\gamma,\epsilon,\delta} \quad (2r_T^3 N_o) \quad (10501)$$

$$\tau^8_{\gamma,\delta,w} = \sum_{\epsilon \in A} \sum_{i \in O} {}^2D^2_{i,w} Y^{2,*}_{i,\delta} \tau^0_{\epsilon,\delta,w} \tau^7_{\epsilon,\gamma,i} \quad (4r_D r_T^3 N_o) \quad (10502)$$

$$\tau^9_{\gamma,\delta,w} = \sum_{\epsilon \in A} Z^*_{\epsilon,\delta} \tau^8_{\gamma,\epsilon,w} \quad (2r_D r_T^3) \quad (10503)$$

$$\tau^{10}_{\gamma,\delta,w} = \sum_{\epsilon \in A} Z_{\gamma,\epsilon} \tau^9_{\epsilon,\delta,w} \quad (2r_D r_T^3) \quad (10504)$$

$$\tau^8_{\gamma,\alpha} = \sum_{a \in V} W^4_{a,\alpha} Y^3_{a,\gamma} \quad (2r_T r_V N_v) \quad (10516)$$

$$\tau^{11}_{\gamma,\delta,w} = \sum_{i \in O} {}^2D^4_{i,w} Y^2_{i,\gamma} Y^{4,*}_{i,\delta} \quad (3r_D r_T^2 N_o) \quad (10505)$$

$$\tau^9_{\gamma,\alpha,i} = \sum_{\delta \in A} Z_{\gamma,\delta} Y^4_{i,\delta} \tau^8_{\delta,\alpha} \quad (3r_T^2 r_V N_o) \quad (10517)$$

$${}^2R^3_{a,\gamma} \leftarrow \sum_{\delta \in A} \sum_{w \in D} \frac{1}{4} {}^2D^3_{a,w} Y^1_{a,\delta} \tau^{10}_{\delta,\gamma,w} \tau^{11}_{\delta,\gamma,w} \quad (4r_D r_T^2 N_v) \quad (10506)$$

$$\tau^{10}_{\gamma,\delta,w,i} = \sum_{\alpha \in B} \tau^7_{\gamma,\alpha} \tau^6_{\delta,\alpha,w} \tau^9_{\gamma,\alpha,i} \quad (3r_D r_T^2 r_V N_o)$$

Raw expression

$$\tau^{11}_{\gamma,\delta,w} = \sum_{i \in O} {}^2D^4_{i,w} Y^{4,*}_{i,\delta} \tau^{10}_{\gamma,\delta,w,i} \quad (3r_D r_T^2 N_o) \quad (10519)$$

$${}^2R^3_{b,\zeta} \leftarrow \sum_{\gamma \in A} \sum_{i \in O} \sum_{j \in O} \sum_{k \in O} \sum_{l \in O} \sum_{a \in V} \sum_{c \in V} \sum_{d \in V} \frac{1}{4} \quad (10507)$$

$$Y^{1,*}_{a,\gamma} \quad Y^{2,*}_{i,\gamma} \quad Z^*_{\gamma,\zeta} \quad Y^{4,*}_{j,\zeta}$$

$${}^2D^{a,i,b,j} \quad {}^2T_{a,k,d,l} \quad {}^2T_{b,j,c,i} \quad V_{k,d,l,c}$$

$${}^2R^3_{a,\gamma} \leftarrow \sum_{\delta \in A} \sum_{w \in D} \frac{1}{4} {}^2D^3_{a,w} Y^1_{a,\delta} \tau^{11}_{\delta,\gamma,w} \quad (3r_D r_T^2 N_v) \quad (10520)$$

Factorized expression

Raw expression

$$\tau^0_{\gamma,\delta,w} = \sum_{a \in V} {}^2D^1_{a,w} Y^1_{a,\gamma} Y^{1,*}_{a,\delta} \quad (3r_D r_T^2 N_v) \quad (10508)$$

$${}^2R^3_{b,\zeta} \leftarrow \sum_{\gamma \in A} \sum_{i \in O} \sum_{j \in O} \sum_{k \in O} \sum_{l \in O} \sum_{a \in V} \sum_{c \in V} \sum_{d \in V} \frac{1}{4} \quad (10521)$$

$$Y^{1,*}_{a,\gamma} \quad Y^{2,*}_{i,\gamma} \quad Z^*_{\gamma,\zeta} \quad Y^{4,*}_{j,\zeta}$$

$${}^2D^{a,i,b,j} \quad {}^2T_{a,k,d,l} \quad {}^2T_{c,i,b,j} \quad V_{k,d,l,c}$$

$$\tau^1_{\gamma,\alpha} = \sum_{i \in O} W^1_{i,\alpha} Y^2_{i,\gamma} \quad (2r_T r_V N_o) \quad (10509)$$

Factorized expression

$$\tau^2_{\gamma,\alpha} = \sum_{a \in V} W^2_{a,\alpha} Y^3_{a,\gamma} \quad (2r_T r_V N_v) \quad (10510)$$

$$\tau^0_{\gamma,\alpha} = \sum_{a \in V} W^4_{a,\alpha} Y^3_{a,\gamma} \quad (2r_T r_V N_v) \quad (10522)$$

$$\tau^3_{\gamma,\alpha,i} = \sum_{\delta \in A} Z_{\gamma,\delta} Y^4_{i,\delta} \tau^2_{\delta,\alpha} \quad (3r_T^2 r_V N_o) \quad (10511)$$

$$\tau^1_{\gamma,\alpha,i} = \sum_{\delta \in A} Z_{\gamma,\delta} Y^4_{i,\delta} \tau^0_{\delta,\alpha} \quad (3r_T^2 r_V N_o) \quad (10523)$$

$$\tau^4_{\gamma,\alpha,w} = \sum_{\delta \in A} \sum_{i \in O} {}^2D^2_{i,w} Y^{2,*}_{i,\gamma} \tau^1_{\delta,\alpha} \tau^0_{\delta,\gamma,w} \tau^3_{\delta,\alpha,i} \quad (5r_D r_T^2 r_V N_o) \quad (10512)$$

$$\tau^4_{\gamma,\delta,\alpha,w} = \sum_{i \in O} {}^2D^4_{i,w} Y^{4,*}_{i,\delta} \tau^1_{\gamma,\alpha,i} \quad (3r_D r_T^2 r_V N_o) \quad (10524)$$

$$\tau^5_{\gamma,\alpha,w} = \sum_{\beta \in B} X_{\beta,\alpha} \tau^4_{\gamma,\beta,w} \quad (2r_D r_T r_V^2) \quad (10513)$$

$$\tau^3_{\gamma,\alpha} = \sum_{a \in V} W^2_{a,\alpha} Y^3_{a,\gamma} \quad (2r_T r_V N_v) \quad (10525)$$

$$\tau^6_{\gamma,\alpha,w} = \sum_{\delta \in A} Z^*_{\delta,\gamma} \tau^5_{\delta,\alpha,w} \quad (2r_D r_T^2 r_V) \quad (10514)$$

$$\tau^4_{\gamma,\alpha,i} = \sum_{\beta \in B} W^1_{i,\beta} X_{\beta,\alpha} \tau^3_{\gamma,\beta} \quad (3r_T r_V^2 N_o) \quad (10526)$$

$$\tau^7_{\gamma,\alpha} = \sum_{i \in O} W^3_{i,\alpha} Y^2_{i,\gamma} \quad (2r_T r_V N_o) \quad (10515)$$

$$\tau^5_{\gamma,\delta,\alpha} = \sum_{i \in O} Y^2_{i,\gamma} \tau^4_{\delta,\alpha,i} \quad (2r_T^2 r_V N_o) \quad (10527)$$

$$\tau_{\gamma,\delta,w}^6 = \sum_{a \in V} {}^2D_{a,w}^1 Y_{a,\gamma}^1 Y_{a,\delta}^{1,*} \quad (3r_D r_T^2 N_v) \quad (10528)$$

$$\tau_{\gamma,\delta,w,i}^7 = \sum_{\epsilon \in A} Y_{i,\epsilon}^{2,*} Z_{\epsilon,\delta}^* \tau_{\gamma,\epsilon,w}^6 \quad (3r_D r_T^3 N_o) \quad (10529)$$

$$\tau_{\gamma,\delta,\epsilon,w}^8 = \sum_{i \in O} {}^2D_{i,w}^2 Y_{i,\delta}^4 \tau_{\gamma,\epsilon,w,i}^7 \quad (3r_D r_T^3 N_o) \quad (10530)$$

$$\tau_{\gamma,\delta,\alpha,w}^9 = \sum_{\epsilon \in A} \tau_{\epsilon,\gamma,\alpha}^5 \tau_{\epsilon,\delta,\alpha,w}^2 \tau_{\epsilon,\gamma,\delta,w}^8 \quad (3r_D r_T^3 r_V) \quad (10531)$$

$$\tau_{\gamma,\delta,w,i}^{10} = \sum_{\alpha \in B} W_{i,\alpha}^3 \tau_{\gamma,\delta,\alpha,w}^9 \quad (2r_D r_T^2 r_V N_o) \quad (10532)$$

$$\tau_{\gamma,\delta,w}^{11} = \sum_{\epsilon \in A} \sum_{i \in O} Y_{i,\gamma}^2 Z_{\gamma,\epsilon} \tau_{\epsilon,\delta,w,i}^{10} \quad (3r_D r_T^3 N_o) \quad (10533)$$

$${}^2R_{a,\gamma}^3 \leftarrow \sum_{\delta \in A} \sum_{w \in D} \frac{1}{4} {}^2D_{a,w}^3 Y_{a,\delta}^1 \tau_{\delta,\gamma,w}^{11} \quad (3r_D r_T^2 N_v) \quad (10534)$$

Raw expression

$${}^2R_{b,\zeta}^3 \leftarrow \sum_{\gamma \in A} \sum_{i \in O} \sum_{j \in O} \sum_{k \in O} \sum_{l \in O} \sum_{a \in V} \sum_{c \in V} \sum_{d \in V} \frac{1}{4} \quad (10535)$$

$$Y_{a,\gamma}^{1,*} Y_{i,\gamma}^{2,*} Z_{\gamma,\zeta}^* Y_{j,\zeta}^{4,*} {}^2D_{a,i,b,j} {}^2T_{a,l,d,i} {}^2T_{b,j,c,k} V_{l,c,k,d}$$

Factorized expression

$$\tau_{\gamma,\alpha}^0 = \sum_{a \in V} W_{a,\alpha}^4 Y_{a,\gamma}^3 \quad (2r_T r_V N_v) \quad (10536)$$

$$\tau_{\gamma,\alpha,i}^1 = \sum_{\delta \in A} Z_{\gamma,\delta} Y_{i,\delta}^4 \tau_{\delta,\alpha}^0 \quad (3r_T^2 r_V N_o) \quad (10537)$$

$$\tau_{\gamma,\delta,\alpha,w}^2 = \sum_{i \in O} {}^2D_{i,w}^4 Y_{i,\delta}^{4,*} \tau_{\gamma,\alpha,i}^1 \quad (3r_D r_T^2 r_V N_o) \quad (10538)$$

$$\tau_{\gamma,\alpha}^3 = \sum_{a \in V} W_{a,\alpha}^2 Y_{a,\gamma}^1 \quad (2r_T r_V N_v) \quad (10539)$$

$$\tau_{\gamma,\alpha,i}^4 = \sum_{\beta \in B} W_{i,\beta}^1 X_{\beta,\alpha} \tau_{\gamma,\beta}^3 \quad (3r_T r_V^2 N_o) \quad (10540)$$

$$\tau_{\gamma,\delta,\alpha}^5 = \sum_{i \in O} Y_{i,\delta}^2 \tau_{\gamma,\alpha,i}^4 \quad (2r_T^2 r_V N_o) \quad (10541)$$

$$\tau_{\gamma,\delta,w}^6 = \sum_{a \in V} {}^2D_{a,w}^1 Y_{a,\gamma}^1 Y_{a,\delta}^{1,*} \quad (3r_D r_T^2 N_v) \quad (10542)$$

$$\tau_{\gamma,\delta,w,i}^7 = \sum_{\epsilon \in A} Y_{i,\epsilon}^{2,*} Z_{\epsilon,\delta}^* \tau_{\gamma,\epsilon,w}^6 \quad (3r_D r_T^3 N_o) \quad (10543)$$

$$\tau_{\gamma,\delta,\epsilon,w}^8 = \sum_{i \in O} {}^2D_{i,w}^2 Y_{i,\delta}^2 \tau_{\gamma,\epsilon,w,i}^7 \quad (3r_D r_T^3 N_o) \quad (10544)$$

$$\tau_{\gamma,\delta,\alpha,w}^9 = \sum_{\epsilon \in A} \tau_{\gamma,\epsilon,\alpha}^5 \tau_{\epsilon,\delta,\alpha,w}^2 \tau_{\epsilon,\gamma,\delta,w}^8 \quad (3r_D r_T^3 r_V) \quad (10545)$$

$$\tau_{\gamma,\delta,w,i}^{10} = \sum_{\alpha \in B} W_{i,\alpha}^3 \tau_{\gamma,\delta,\alpha,w}^9 \quad (2r_D r_T^2 r_V N_o) \quad (10546)$$

$$\tau_{\gamma,\delta,w}^{11} = \sum_{\epsilon \in A} \sum_{i \in O} Z_{\epsilon,\gamma} Y_{i,\gamma}^4 \tau_{\epsilon,\delta,w,i}^{10} \quad (3r_D r_T^3 N_o) \quad (10547)$$

$${}^2R_{a,\gamma}^3 \leftarrow \sum_{\delta \in A} \sum_{w \in D} \frac{1}{4} {}^2D_{a,w}^3 Y_{a,\delta}^3 \tau_{\delta,\gamma,w}^{11} \quad (3r_D r_T^2 N_v) \quad (10548)$$

Raw expression

$${}^2R_{b,\zeta}^3 \leftarrow \sum_{\gamma \in A} \sum_{i \in O} \sum_{j \in O} \sum_{k \in O} \sum_{l \in O} \sum_{a \in V} \sum_{c \in V} \sum_{d \in V} \frac{1}{4} \quad (10549)$$

$$Y_{a,\gamma}^{1,*} Y_{i,\gamma}^{2,*} Z_{\gamma,\zeta}^* Y_{j,\zeta}^{4,*} {}^2D_{a,i,b,j} {}^2T_{a,l,d,i} {}^2T_{b,k,c,j} V_{l,d,k,c}$$

Factorized expression

$$\tau_{\gamma,\delta,w}^0 = \sum_{a \in V} {}^2D_{a,w}^1 Y_{a,\gamma}^1 Y_{a,\delta}^{1,*} \quad (3r_D r_T^2 N_v) \quad (10550)$$

$$\tau_{\gamma,\delta,w}^1 = \sum_{i \in O} {}^2D_{i,w}^2 Y_{i,\gamma}^2 Y_{i,\delta}^{2,*} \quad (3r_D r_T^2 N_o) \quad (10551)$$

$$\tau_{\gamma,\delta,w}^2 = \sum_{\epsilon \in A} Z_{\epsilon,\delta}^* \tau_{\gamma,\epsilon,w}^0 \tau_{\gamma,\epsilon,w}^1 \quad (3r_D r_T^3) \quad (10552)$$

$$\tau_{\gamma,\delta,w}^3 = \sum_{\epsilon \in A} Z_{\epsilon,\gamma} \tau_{\epsilon,\delta,w}^2 \quad (2r_D r_T^3) \quad (10553)$$

$$\tau_{\gamma,\alpha}^4 = \sum_{a \in V} W_{a,\alpha}^4 Y_{a,\gamma}^3 \quad (2r_T r_V N_v) \quad (10554)$$

$$\tau_{\gamma,\alpha,i}^5 = \sum_{\beta \in B} X_{\alpha,\beta} W_{i,\beta}^3 \tau_{\gamma,\beta}^4 \quad (3r_T r_V^2 N_o) \quad (10555)$$

$$\tau_{\gamma,\alpha}^6 = \sum_{i \in O} W_{i,\alpha}^1 Y_{i,\gamma}^4 \quad (2r_T r_V N_o) \quad (10556)$$

$$\tau_{\gamma,\alpha}^7 = \sum_{a \in V} W_{a,\alpha}^2 Y_{a,\gamma}^1 \quad (2r_T r_V N_v) \quad (10557)$$

$$\tau_{\gamma,\delta,i}^8 = \sum_{\alpha \in B} \tau_{\delta,\alpha}^6 \tau_{\gamma,\alpha}^7 \tau_{\delta,\alpha,i}^5 \quad (3r_T^2 r_V N_o) \quad (10558)$$

$$\tau_{\gamma,\delta,\epsilon}^9 = \sum_{i \in O} Z_{\gamma,\delta} Y_{i,\delta}^4 \tau_{\gamma,\epsilon,i}^8 \quad (3r_T^3 N_o) \quad (10559)$$

$$\tau_{\gamma,\delta,i}^{10} = \sum_{\epsilon \in A} Y_{i,\epsilon}^2 \tau_{\epsilon,\gamma,\delta}^9 \quad (2r_T^3 N_o) \quad (10560)$$

$$\tau_{\gamma,\delta,w}^{11} = \sum_{\epsilon \in A} \sum_{i \in O} {}^2D_{i,w}^4 Y_{i,\delta}^{4,*} \tau_{\gamma,\epsilon,i}^{10} \tau_{\epsilon,\delta,w}^3 \quad (4r_D r_T^3 N_o) \quad (10561)$$

$${}^2R_{a,\gamma}^3 \leftarrow \sum_{\delta \in A} \sum_{w \in D} \frac{1}{4} {}^2D_{a,w}^3 Y_{a,\delta}^3 \tau_{\delta,\gamma,w}^{11} \quad (3r_D r_T^2 N_v) \quad (10562)$$

Raw expression

$${}^2R_{b,\zeta}^3 \leftarrow \sum_{\gamma \in A} \sum_{i \in O} \sum_{j \in O} \sum_{k \in O} \sum_{l \in O} \sum_{a \in V} \sum_{c \in V} \sum_{d \in V} \frac{1}{4} \quad (10563)$$

$$Y_{a,\gamma}^{1,*} Y_{i,\gamma}^{2,*} Z_{\gamma,\zeta}^* Y_{j,\zeta}^{4,*} {}^2D_{a,i,b,j} {}^2T_{a,l,d,i} {}^2T_{c,j,b,k} V_{l,d,k,c}$$

Factorized expression

$$\tau_{\gamma,\delta,w}^0 = \sum_{a \in V} {}^2D_{a,w}^1 Y_{a,\gamma}^1 Y_{a,\delta}^{1,*} \quad (3r_D r_T^2 N_v) \quad (10564)$$

$$\tau_{\gamma,\alpha}^1 = \sum_{a \in V} W_{a,\alpha}^2 Y_{a,\gamma}^1 \quad (2r_T r_V N_v) \quad (10565)$$

$$\tau_{\gamma,\alpha,i}^2 = \sum_{\beta \in B} W_{i,\beta}^1 X_{\beta,\alpha} \tau_{\gamma,\beta}^1 \quad (3r_T r_V^2 N_o) \quad (10566)$$

$$\tau_{\gamma,\alpha}^3 = \sum_{i \in O} W_{i,\alpha}^3 Y_{i,\gamma}^2 \quad (2r_T r_V N_o) \quad (10567)$$

$$\tau_{\gamma,\alpha}^4 = \sum_{a \in V} W_{a,\alpha}^4 Y_{a,\gamma}^3 \quad (2r_T r_V N_v) \quad (10568)$$

$$\tau_{\gamma,\delta,i}^5 = \sum_{\alpha \in B} \tau_{\gamma,\alpha}^3 \tau_{\delta,\alpha}^4 \tau_{\gamma,\alpha,i}^2 \quad (3r_T^2 r_V N_o) \quad (10569)$$

$$\tau_{\gamma,\delta,\epsilon}^6 = \sum_{i \in O} Y_{i,\delta}^2 Z_{\delta,\epsilon} \tau_{\gamma,\epsilon,i}^5 \quad (3r_T^3 N_o) \quad (10570)$$

$$\tau_{\gamma,\delta,i}^7 = \sum_{\epsilon \in A} Y_{i,\epsilon}^4 \tau_{\gamma,\delta,\epsilon}^6 \quad (2r_T^3 N_o) \quad (10571)$$

$$\tau_{\gamma,\delta,w}^8 = \sum_{\epsilon \in A} \sum_{i \in O} {}^2D_{i,w}^2 Y_{i,\delta}^{2,*} \tau_{\epsilon,\delta,w}^0 \tau_{\gamma,\epsilon,i}^7 \quad (4r_D r_T^3 N_o) \quad (10572)$$

$$\tau_{\gamma,\delta,w}^9 = \sum_{\epsilon \in A} Z_{\epsilon,\delta}^* \tau_{\gamma,\epsilon,w}^8 \quad (2r_D r_T^3) \quad (10573)$$

$$\tau_{\gamma,\delta,w}^{10} = \sum_{\epsilon \in A} Z_{\epsilon,\gamma} \tau_{\epsilon,\delta,w}^9 \quad (2r_D r_T^3) \quad (10574)$$

$$\tau_{\gamma,\delta,w}^{11} = \sum_{i \in O} {}^2D_{i,w}^4 Y_{i,\gamma}^4 Y_{i,\delta}^{4,*} \quad (3r_D r_T^2 N_o) \quad (10575)$$

$${}^2R^3_{a,\gamma} \leftarrow \sum_{\delta \in A} \sum_{w \in D} \frac{1}{4} {}^2D^3_{a,w} Y^3_{a,\delta} \tau^{10}_{\delta,\gamma,w} \tau^{11}_{\delta,\gamma,w} \quad (4r_D r_T^2 N_v) \quad \tau^{11}_{\gamma,\delta,w} = \sum_{\epsilon \in A} Z_{\epsilon,\gamma} \tau^{10}_{\epsilon,\delta,w} \quad (2r_D r_T^3) \quad (10589)$$

$$(10576)$$

Raw expression

$${}^2R^3_{a,\gamma} \leftarrow \sum_{\delta \in A} \sum_{w \in D} \frac{1}{4} {}^2D^3_{a,w} Y^3_{a,\delta} \tau^0_{\delta,\gamma,w} \tau^{11}_{\delta,\gamma,w} \quad (4r_D r_T^2 N_v) \quad (10590)$$

$${}^2R^3_{b,\zeta} \leftarrow \sum_{\gamma \in A} \sum_{i \in O} \sum_{j \in O} \sum_{k \in O} \sum_{l \in O} \sum_{a \in V} \sum_{c \in V} \sum_{d \in V} \frac{1}{4} \quad (10577)$$

$$Y^{1,*}_{a,\gamma} \quad Y^{2,*}_{i,\gamma} \quad Z^*_{\gamma,\zeta} \quad Y^{4,*}_{j,\zeta}$$

$${}^2D^{a,i,b,j} \quad {}^2T_{a,l,d,i} \quad {}^2T_{c,k,b,j} \quad V_{l,c,k,d}$$

Factorized expression

Raw expression

$${}^2R^3_{b,\zeta} \leftarrow \sum_{\gamma \in A} \sum_{i \in O} \sum_{j \in O} \sum_{k \in O} \sum_{l \in O} \sum_{a \in V} \sum_{c \in V} \sum_{d \in V} \frac{1}{4} \quad (10591)$$

$$Y^{1,*}_{a,\gamma} \quad Y^{2,*}_{i,\gamma} \quad Z^*_{\gamma,\zeta} \quad Y^{4,*}_{j,\zeta}$$

$${}^2D^{a,i,b,j} \quad {}^2T_{a,l,d,j} \quad {}^2T_{b,k,c,i} \quad V_{l,c,k,d}$$

Factorized expression

$$\tau^0_{\gamma,\delta,w} = \sum_{i \in O} {}^2D^4_{i,w} Y^4_{i,\gamma} Y^{4,*}_{i,\delta} \quad (3r_D r_T^2 N_o) \quad (10578)$$

$$\tau^1_{\gamma,\delta,w} = \sum_{i \in O} {}^2D^2_{i,w} Y^2_{i,\gamma} Y^{2,*}_{i,\delta} \quad (3r_D r_T^2 N_o) \quad (10579)$$

$$\tau^0_{\gamma,\delta,w} = \sum_{i \in O} {}^2D^4_{i,w} Y^4_{i,\gamma} Y^{4,*}_{i,\delta} \quad (3r_D r_T^2 N_o) \quad (10592)$$

$$\tau^2_{\gamma,\alpha} = \sum_{a \in V} W^2_{a,\alpha} Y^3_{a,\gamma} \quad (2r_T r_V N_v) \quad (10580)$$

$$\tau^1_{\gamma,\delta,w} = \sum_{a \in V} {}^2D^1_{a,w} Y^1_{a,\gamma} Y^{1,*}_{a,\delta} \quad (3r_D r_T^2 N_v) \quad (10593)$$

$$\tau^3_{\gamma,\alpha,i} = \sum_{\beta \in B} W^1_{i,\beta} X_{\beta,\alpha} \tau^2_{\gamma,\beta} \quad (3r_T r_V^2 N_o) \quad (10581)$$

$$\tau^2_{\gamma,\delta,w} = \sum_{i \in O} {}^2D^2_{i,w} Y^2_{i,\gamma} Y^{2,*}_{i,\delta} \quad (3r_D r_T^2 N_o) \quad (10594)$$

$$\tau^4_{\gamma,\alpha} = \sum_{i \in O} W^3_{i,\alpha} Y^4_{i,\gamma} \quad (2r_T r_V N_o) \quad (10582)$$

$$\tau^3_{\gamma,\delta,w} = \sum_{\epsilon \in A} Z^*_{\epsilon,\delta} \tau^1_{\gamma,\epsilon,w} \tau^2_{\gamma,\epsilon,w} \quad (3r_D r_T^3) \quad (10595)$$

$$\tau^5_{\gamma,\alpha} = \sum_{\delta \in A} \sum_{i \in O} Y^2_{i,\gamma} Z_{\gamma,\delta} \tau^4_{\delta,\alpha} \tau^3_{\delta,\alpha,i} \quad (4r_T^2 r_V N_o) \quad (10583)$$

$$\tau^4_{\gamma,\delta,w} = \sum_{\epsilon \in A} Z_{\epsilon,\gamma} \tau^3_{\epsilon,\delta,w} \quad (2r_D r_T^3) \quad (10596)$$

$$\tau^6_{\gamma,a} = \sum_{\alpha \in B} W^4_{a,\alpha} \tau^5_{\gamma,\alpha} \quad (2r_T r_V N_v) \quad (10584)$$

$$\tau^5_{\gamma,\alpha} = \sum_{a \in V} W^4_{a,\alpha} Y^1_{a,\gamma} \quad (2r_T r_V N_v) \quad (10597)$$

$$\tau^7_{\gamma,\delta} = \sum_{a \in V} Y^1_{a,\gamma} \tau^6_{\delta,a} \quad (2r_T^2 N_v) \quad (10585)$$

$$\tau^6_{\gamma,\alpha,i} = \sum_{\beta \in B} X_{\alpha,\beta} W^3_{i,\beta} \tau^5_{\gamma,\beta} \quad (3r_T r_V^2 N_o) \quad (10598)$$

$$\tau^8_{\gamma,a} = \sum_{\delta \in A} Y^1_{a,\delta} \tau^7_{\gamma,\delta} \quad (2r_T^2 N_v) \quad (10586)$$

$$\tau^7_{\gamma,\alpha} = \sum_{i \in O} W^1_{i,\alpha} Y^2_{i,\gamma} \quad (2r_T r_V N_o) \quad (10599)$$

$$\tau^9_{\gamma,\delta,w} = \sum_{a \in V} {}^2D^1_{a,w} Y^{1,*}_{a,\delta} \tau^8_{\gamma,a} \quad (3r_D r_T^2 N_v) \quad (10587)$$

$$\tau^8_{\gamma,\alpha} = \sum_{\delta \in A} \sum_{i \in O} Z_{\delta,\gamma} Y^4_{i,\gamma} \tau^7_{\delta,\alpha} \tau^6_{\delta,\alpha,i} \quad (4r_T^2 r_V N_o) \quad (10600)$$

$$\tau^{10}_{\gamma,\delta,w} = \sum_{\epsilon \in A} Z^*_{\epsilon,\delta} \tau^1_{\gamma,\epsilon,w} \tau^9_{\gamma,\epsilon,w} \quad (3r_D r_T^3) \quad (10588)$$

$$\tau^9_{\gamma,a} = \sum_{\alpha \in B} W^2_{a,\alpha} \tau^8_{\gamma,\alpha} \quad (2r_T r_V N_v) \quad (10601)$$



$$\tau_{a,b}^{10} = \sum_{\gamma \in A} Y_{b,\gamma}^3 \tau_{\gamma,a}^9 \quad (2r_T N_v^2) \quad (10602)$$

$$\tau_{\gamma,\alpha}^9 = \sum_{i \in O} W_{i,\alpha}^3 Y_{i,\gamma}^4 \quad (2r_T r_V N_o) \quad (10615)$$

$$\tau_{\gamma,a}^{11} = \sum_{b \in V} Y_{b,\gamma}^3 \tau_{b,a}^{10} \quad (2r_T N_v^2) \quad (10603)$$

$$\tau_{\gamma,\delta,w,i}^{10} = \sum_{\alpha \in B} \tau_{\gamma,\alpha}^9 \tau_{\delta,\alpha,w}^6 \tau_{\gamma,\alpha,i}^8 \quad (3r_D r_T^2 r_V N_o) \quad (10616)$$

$${}^2R_{a,\gamma}^3 \leftarrow \sum_{\delta \in A} \sum_{w \in D} \frac{1}{4} {}^2D_{a,w}^3 \tau_{\delta,a}^{11} \tau_{\delta,\gamma,w}^0 \tau_{\delta,\gamma,w}^4 \quad (4r_D r_T^2 N_v) \quad (10604)$$

$$\tau_{\gamma,\delta,w}^{11} = \sum_{i \in O} {}^2D_{i,w}^4 Y_{i,\delta}^{4,*} \tau_{\gamma,\delta,w,i}^{10} \quad (3r_D r_T^2 N_o) \quad (10617)$$

Raw expression

$${}^2R_{b,\zeta}^3 \leftarrow \sum_{\gamma \in A} \sum_{i \in O} \sum_{j \in O} \sum_{k \in O} \sum_{l \in O} \sum_{a \in V} \sum_{c \in V} \sum_{d \in V} \frac{1}{4} \quad (10605)$$

$$Y_{a,\gamma}^{1,*} Y_{i,\gamma}^{2,*} Z_{\gamma,\zeta}^* Y_{j,\zeta}^{4,*} {}^2D_{a,i,b,j} {}^2T_{a,l,d,j} {}^2T_{c,i,b,k} V_{l,c,k,d}$$

$${}^2R_{a,\gamma}^3 \leftarrow \sum_{\delta \in A} \sum_{w \in D} \frac{1}{4} {}^2D_{a,w}^3 Y_{a,\delta}^3 \tau_{\delta,\gamma,w}^{11} \quad (3r_D r_T^2 N_v) \quad (10618)$$

Raw expression

Factorized expression

$$\tau_{\gamma,\delta,w}^0 = \sum_{a \in V} {}^2D_{a,w}^1 Y_{a,\gamma}^1 Y_{a,\delta}^{1,*} \quad (3r_D r_T^2 N_v) \quad (10606)$$

$${}^2R_{b,\zeta}^3 \leftarrow \sum_{\gamma \in A} \sum_{i \in O} \sum_{j \in O} \sum_{k \in O} \sum_{l \in O} \sum_{a \in V} \sum_{c \in V} \sum_{d \in V} \frac{1}{4} \quad (10619)$$

$$Y_{a,\gamma}^{1,*} Y_{i,\gamma}^{2,*} Z_{\gamma,\zeta}^* Y_{j,\zeta}^{4,*} {}^2D_{a,i,b,j} {}^2T_{b,j,a,k} {}^2T_{c,i,d,l} V_{k,d,l,c}$$

Factorized expression

$$\tau_{\gamma,\alpha}^1 = \sum_{i \in O} W_{i,\alpha}^1 Y_{i,\gamma}^2 \quad (2r_T r_V N_o) \quad (10607)$$

$$\tau_{\gamma,\delta,w}^0 = \sum_{a \in V} {}^2D_{a,w}^1 Y_{a,\gamma}^3 Y_{a,\delta}^{1,*} \quad (3r_D r_T^2 N_v) \quad (10620)$$

$$\tau_{\gamma,\alpha}^2 = \sum_{a \in V} W_{a,\alpha}^2 Y_{a,\gamma}^3 \quad (2r_T r_V N_v) \quad (10608)$$

$$\tau_{\gamma,\alpha}^1 = \sum_{a \in V} W_{a,\alpha}^2 Y_{a,\gamma}^1 \quad (2r_T r_V N_v) \quad (10621)$$

$$\tau_{\gamma,\alpha,i}^3 = \sum_{\delta \in A} Z_{\gamma,\delta} Y_{i,\delta}^4 \tau_{\delta,\alpha}^2 \quad (3r_T^2 r_V N_o) \quad (10609)$$

$$\tau_{\gamma,\alpha,w}^4 = \sum_{\delta \in A} \sum_{i \in O} {}^2D_{i,w}^2 Y_{i,\gamma}^{2,*} \tau_{\delta,\alpha}^1 \tau_{\delta,\gamma,w}^0 \tau_{\delta,\alpha,i}^3 \quad (5r_D r_T^2 r_V N_o) \quad (10610)$$

$$\tau_{\gamma,\alpha,i}^2 = \sum_{\delta \in A} Y_{i,\delta}^2 Z_{\delta,\gamma} \tau_{\delta,\alpha}^1 \quad (3r_T^2 r_V N_o) \quad (10622)$$

$$\tau_{\gamma,\alpha,w}^5 = \sum_{\beta \in B} X_{\beta,\alpha} \tau_{\gamma,\beta,w}^4 \quad (2r_D r_T r_V^2) \quad (10611)$$

$$\tau_{\gamma,\alpha}^3 = \sum_{i \in O} W_{i,\alpha}^1 Y_{i,\gamma}^4 \quad (2r_T r_V N_o) \quad (10623)$$

$$\tau_{\gamma,\alpha,w}^6 = \sum_{\delta \in A} Z_{\delta,\gamma}^* \tau_{\delta,\alpha,w}^5 \quad (2r_D r_T^2 r_V) \quad (10612)$$

$$\tau_{\gamma,\alpha,w}^4 = \sum_{\delta \in A} \sum_{i \in O} {}^2D_{i,w}^2 Y_{i,\gamma}^{2,*} \tau_{\delta,\alpha}^3 \tau_{\delta,\gamma,w}^0 \tau_{\delta,\alpha,i}^2 \quad (5r_D r_T^2 r_V N_o) \quad (10624)$$

$$\tau_{\gamma,\alpha}^7 = \sum_{a \in V} W_{a,\alpha}^4 Y_{a,\gamma}^1 \quad (2r_T r_V N_v) \quad (10613)$$

$$\tau_{\gamma,\alpha,w}^5 = \sum_{\beta \in B} X_{\beta,\alpha} \tau_{\gamma,\beta,w}^4 \quad (2r_D r_T r_V^2) \quad (10625)$$

$$\tau_{\gamma,\alpha,i}^8 = \sum_{\delta \in A} Y_{i,\delta}^2 Z_{\delta,\gamma} \tau_{\delta,\alpha}^7 \quad (3r_T^2 r_V N_o) \quad (10614)$$

$$\tau_{\gamma,\alpha,w}^6 = \sum_{\delta \in A} Z_{\delta,\gamma}^* \tau_{\delta,\alpha,w}^5 \quad (2r_D r_T^2 r_V) \quad (10626)$$

$$\tau^7_{\gamma,\alpha} = \sum_{i \in O} W^3_{i,\alpha} Y^2_{i,\gamma} \quad (2r_T r_V N_o) \quad (10627)$$

$$\tau^8_{\gamma,\alpha} = \sum_{a \in V} W^4_{a,\alpha} Y^3_{a,\gamma} \quad (2r_T r_V N_v) \quad (10628)$$

$$\tau^9_{\gamma,\alpha,i} = \sum_{\delta \in A} Z_{\gamma,\delta} Y^4_{i,\delta} \tau^8_{\delta,\alpha} \quad (3r_T^2 r_V N_o) \quad (10629)$$

$$\tau^{10}_{\gamma,\delta,w,i} = \sum_{\alpha \in B} \tau^7_{\gamma,\alpha} \tau^6_{\delta,\alpha,w} \tau^9_{\gamma,\alpha,i} \quad (3r_D r_T^2 r_V N_o) \quad (10630)$$

$$\tau^{11}_{\gamma,\delta,w} = \sum_{i \in O} {}^2D^4_{i,w} Y^{4,*}_{i,\delta} \tau^{10}_{\gamma,\delta,w,i} \quad (3r_D r_T^2 N_o) \quad (10631)$$

$${}^2R^3_{a,\gamma} \leftarrow \sum_{\delta \in A} \sum_{w \in D} \frac{1}{4} {}^2D^3_{a,w} Y^1_{a,\delta} \tau^{11}_{\delta,\gamma,w} \quad (3r_D r_T^2 N_v) \quad (10632)$$

Raw expression

$${}^2R^3_{b,\zeta} \leftarrow \sum_{\gamma \in A} \sum_{i \in O} \sum_{j \in O} \sum_{k \in O} \sum_{l \in O} \sum_{a \in V} \sum_{c \in V} \sum_{d \in V} \frac{1}{4} \quad (10633)$$

$$Y^{1,*}_{a,\gamma} \quad Y^{2,*}_{i,\gamma} \quad Z^*_{\gamma,\zeta} \quad Y^{4,*}_{j,\zeta}$$

$${}^2D^{a,i,b,j} \quad {}^2T_{b,j,a,k} \quad {}^2T_{c,l,d,i} \quad V_{k,c,l,d}$$

Factorized expression

$$\tau^0_{\gamma,\delta,w} = \sum_{i \in O} {}^2D^4_{i,w} Y^2_{i,\gamma} Y^{4,*}_{i,\delta} \quad (3r_D r_T^2 N_o) \quad (10634)$$

$$\tau^1_{\gamma,\delta,w} = \sum_{a \in V} {}^2D^1_{a,w} Y^3_{a,\gamma} Y^{1,*}_{a,\delta} \quad (3r_D r_T^2 N_v) \quad (10635)$$

$$\tau^2_{\gamma,\alpha} = \sum_{a \in V} W^2_{a,\alpha} Y^1_{a,\gamma} \quad (2r_T r_V N_v) \quad (10636)$$

$$\tau^3_{\gamma,\alpha,i} = \sum_{\beta \in B} W^1_{i,\beta} X_{\beta,\alpha} \tau^2_{\gamma,\beta} \quad (3r_T r_V^2 N_o) \quad (10637)$$

$$\tau^4_{\gamma,\alpha} = \sum_{i \in O} W^3_{i,\alpha} Y^2_{i,\gamma} \quad (2r_T r_V N_o) \quad (10638)$$

$$\tau^5_{\gamma,\alpha} = \sum_{a \in V} W^4_{a,\alpha} Y^3_{a,\gamma} \quad (2r_T r_V N_v) \quad (10639)$$

$$\tau^6_{\gamma,\delta,i} = \sum_{\alpha \in B} \tau^4_{\gamma,\alpha} \tau^5_{\delta,\alpha} \tau^3_{\gamma,\alpha,i} \quad (3r_T^2 r_V N_o) \quad (10640)$$

$$\tau^7_{\gamma,i} = \sum_{\delta \in A} Z_{\delta,\gamma} \tau^6_{\delta,\gamma,i} \quad (2r_T^2 N_o) \quad (10641)$$

$$\tau^8_{i,j} = \sum_{\gamma \in A} Y^4_{j,\gamma} \tau^7_{\gamma,i} \quad (2r_T N_o^2) \quad (10642)$$

$$\tau^9_{\gamma,i} = \sum_{j \in O} Y^4_{j,\gamma} \tau^8_{j,i} \quad (2r_T N_o^2) \quad (10643)$$

$$\tau^{10}_{\gamma,\delta,w} = \sum_{i \in O} {}^2D^2_{i,w} Y^{2,*}_{i,\delta} \tau^9_{\gamma,i} \quad (3r_D r_T^2 N_o) \quad (10644)$$

$$\tau^{11}_{\gamma,\delta,w} = \sum_{\epsilon \in A} Z^*_{\epsilon,\delta} \tau^1_{\gamma,\epsilon,w} \tau^{10}_{\gamma,\epsilon,w} \quad (3r_D r_T^3) \quad (10645)$$

$$\tau^{12}_{\gamma,\delta,w} = \sum_{\epsilon \in A} Z_{\gamma,\epsilon} \tau^{11}_{\epsilon,\delta,w} \quad (2r_D r_T^3) \quad (10646)$$

$${}^2R^3_{a,\gamma} \leftarrow \sum_{\delta \in A} \sum_{w \in D} \frac{1}{4} {}^2D^3_{a,w} Y^1_{a,\delta} \tau^0_{\delta,\gamma,w} \tau^{12}_{\delta,\gamma,w} \quad (4r_D r_T^2 N_v) \quad (10647)$$

Raw expression

$${}^2R^3_{b,\zeta} \leftarrow \sum_{\gamma \in A} \sum_{i \in O} \sum_{j \in O} \sum_{k \in O} \sum_{l \in O} \sum_{a \in V} \sum_{c \in V} \sum_{d \in V} \frac{1}{4} \quad (10648)$$

$$Y^{1,*}_{a,\gamma} \quad Y^{2,*}_{i,\gamma} \quad Z^*_{\gamma,\zeta} \quad Y^{4,*}_{j,\zeta}$$

$${}^2D^{a,i,b,j} \quad {}^2T_{b,j,c,i} \quad {}^2T_{d,k,a,l} \quad V_{k,c,l,d}$$

Factorized expression

$$\tau^0_{\gamma,\delta,w} = \sum_{a \in V} {}^2D^1_{a,w} Y^3_{a,\gamma} Y^{1,*}_{a,\delta} \quad (3r_D r_T^2 N_v) \quad (10649)$$

$$\tau^1_{\gamma,\delta,w,i} = \sum_{\epsilon \in A} Y^{2,*}_{i,\epsilon} Z^*_{\epsilon,\delta} \tau^0_{\gamma,\epsilon,w} \quad (3r_D r_T^3 N_o) \quad (10650)$$

$$\tau^2_{\gamma,\alpha} = \sum_{a \in V} W^2_{a,\alpha} Y^1_{a,\gamma} \quad (2r_T r_V N_v) \quad (10651)$$

$$\tau^3_{\gamma,\alpha,i} = \sum_{\beta \in B} W^1_{i,\beta} X_{\beta,\alpha} \tau^2_{\gamma,\beta} \quad (3r_T r_V^2 N_o) \quad (10652)$$

$$\tau^2_{\gamma,\alpha} = \sum_{i \in O} W^3_{i,\alpha} Y^2_{i,\gamma} \quad (2r_T r_V N_o) \quad (10664)$$

$$\tau^4_{\gamma,\alpha} = \sum_{a \in V} W^4_{a,\alpha} Y^3_{a,\gamma} \quad (2r_T r_V N_v) \quad (10653)$$

$$\tau^3_{\gamma,\alpha} = \sum_{a \in V} W^4_{a,\alpha} Y^3_{a,\gamma} \quad (2r_T r_V N_v) \quad (10665)$$

$$\tau^5_{\gamma,\alpha,i} = \sum_{\delta \in A} Z_{\gamma,\delta} Y^4_{i,\delta} \tau^4_{\delta,\alpha} \quad (3r_T^2 r_V N_o) \quad (10654)$$

$$\tau^4_{\gamma,\delta,i} = \sum_{\alpha \in B} \tau^2_{\gamma,\alpha} \tau^3_{\delta,\alpha} \tau^1_{\gamma,\alpha,i} \quad (3r_T^2 r_V N_o) \quad (10666)$$

$$\tau^6_{\gamma,i,j,k} = \sum_{\alpha \in B} W^3_{j,\alpha} \tau^3_{\gamma,\alpha,i} \tau^5_{\gamma,\alpha,k} \quad (3r_T r_V N_o^3) \quad (10655)$$

$$\tau^5_{\gamma,i} = \sum_{\delta \in A} Z_{\delta,\gamma} \tau^4_{\delta,\gamma,i} \quad (2r_T^2 N_o) \quad (10667)$$

$$\tau^7_{i,j,k,l} = \sum_{\gamma \in A} Y^2_{k,\gamma} \tau^6_{\gamma,i,j,l} \quad (2r_T N_o^4) \quad (10656)$$

$$\tau^6_{i,j} = \sum_{\gamma \in A} Y^4_{j,\gamma} \tau^5_{\gamma,i} \quad (2r_T N_o^2) \quad (10668)$$

$$\tau^8_{\gamma,i,j,k} = \sum_{l \in O} Y^4_{l,\gamma} \tau^7_{i,l,j,k} \quad (2r_T N_o^4) \quad (10657)$$

$$\tau^7_{\gamma,i} = \sum_{j \in O} Y^2_{j,\gamma} \tau^6_{j,i} \quad (2r_T N_o^2) \quad (10669)$$

$$\tau^9_{\gamma,\delta,w,i} = \sum_{j \in O} \sum_{k \in O} {}^2D^2_{j,w} {}^2D^4_{k,w} Y^{4,*}_{k,\delta} \tau^1_{\gamma,\delta,w,j} \tau^8_{\gamma,i,k,j} \quad (5r_D r_T^2 N_o^3) \quad (10658)$$

$$\tau^8_{\gamma,\delta,w} = \sum_{i \in O} {}^2D^4_{i,w} Y^{4,*}_{i,\delta} \tau^7_{\gamma,i} \quad (3r_D r_T^2 N_o) \quad (10670)$$

$$\tau^9_{\gamma,\delta,w} = \sum_{a \in V} {}^2D^1_{a,w} Y^3_{a,\gamma} Y^{1,*}_{a,\delta} \quad (3r_D r_T^2 N_v) \quad (10671)$$

$$\tau^{10}_{\gamma,\delta,w} = \sum_{\epsilon \in A} \sum_{i \in O} Y^2_{i,\gamma} Z_{\gamma,\epsilon} \tau^9_{\epsilon,\delta,w,i} \quad (3r_D r_T^3 N_o) \quad (10659)$$

$$\tau^{10}_{\gamma,\delta,w} = \sum_{i \in O} {}^2D^2_{i,w} Y^4_{i,\gamma} Y^{2,*}_{i,\delta} \quad (3r_D r_T^2 N_o) \quad (10672)$$

$${}^2R^3_{a,\gamma} \leftarrow \sum_{\delta \in A} \sum_{w \in D} \frac{1}{4} {}^2D^3_{a,w} Y^1_{a,\delta} \tau^{10}_{\delta,\gamma,w} \quad (3r_D r_T^2 N_v) \quad (10660)$$

$$\tau^{11}_{\gamma,\delta,w} = \sum_{\epsilon \in A} Z^*_{\epsilon,\delta} \tau^{10}_{\gamma,\epsilon,w} \tau^9_{\gamma,\epsilon,w} \quad (3r_D r_T^3) \quad (10673)$$

Raw expression

$${}^2R^3_{b,\zeta} \leftarrow \sum_{\gamma \in A} \sum_{i \in O} \sum_{j \in O} \sum_{k \in O} \sum_{l \in O} \sum_{a \in V} \sum_{c \in V} \sum_{d \in V} \frac{1}{4} Y^{1,*}_{a,\gamma} Y^{2,*}_{i,\gamma} Z^*_{\gamma,\zeta} Y^{4,*}_{j,\zeta} {}^2D^{a,i,b,j} {}^2T_{b,j,c,k} {}^2T_{d,i,a,l} V_{l,c,k,d} \quad (10661)$$

$$\tau^{12}_{\gamma,\delta,w} = \sum_{\epsilon \in A} Z_{\gamma,\epsilon} \tau^{11}_{\epsilon,\delta,w} \quad (2r_D r_T^3) \quad (10674)$$

$${}^2R^3_{a,\gamma} \leftarrow \sum_{\delta \in A} \sum_{w \in D} \frac{1}{4} {}^2D^3_{a,w} Y^1_{a,\delta} \tau^{12}_{\delta,\gamma,w} \tau^8_{\delta,\gamma,w} \quad (4r_D r_T^2 N_v) \quad (10675)$$

Factorized expression

$$\tau^0_{\gamma,\alpha} = \sum_{a \in V} W^2_{a,\alpha} Y^1_{a,\gamma} \quad (2r_T r_V N_v) \quad (10662)$$

Raw expression

$$\tau^1_{\gamma,\alpha,i} = \sum_{\beta \in B} W^1_{i,\beta} X_{\beta,\alpha} \tau^0_{\gamma,\beta} \quad (3r_T r_V^2 N_o) \quad (10663)$$

$${}^2R^3_{b,\zeta} \leftarrow \sum_{\gamma \in A} \sum_{i \in O} \sum_{j \in O} \sum_{k \in O} \sum_{l \in O} \sum_{a \in V} \sum_{c \in V} \sum_{d \in V} \frac{1}{4} Y^{1,*}_{a,\gamma} Y^{2,*}_{i,\gamma} Z^*_{\gamma,\zeta} Y^{4,*}_{j,\zeta} {}^2D^{a,i,b,j} {}^2T_{b,k,a,i} {}^2T_{c,j,d,l} V_{k,d,l,c} \quad (10676)$$

Factorized expression

$$\tau_{\gamma,\delta,w}^0 = \sum_{a \in V} {}^2D_{a,w}^1 Y_{a,\gamma}^3 Y_{a,\delta}^{1,*} \quad (3r_D r_T^2 N_v) \quad (10677)$$

$$\tau_{\gamma,\alpha}^1 = \sum_{a \in V} W_{a,\alpha}^2 Y_{a,\gamma}^3 \quad (2r_T r_V N_v) \quad (10678)$$

$$\tau_{\gamma,\alpha,i}^2 = \sum_{\beta \in B} W_{i,\beta}^1 X_{\beta,\alpha} \tau_{\gamma,\beta}^1 \quad (3r_T r_V^2 N_o) \quad (10679)$$

$$\tau_{\gamma,\alpha}^3 = \sum_{i \in O} W_{i,\alpha}^3 Y_{i,\gamma}^4 \quad (2r_T r_V N_o) \quad (10680)$$

$$\tau_{\gamma,\alpha}^4 = \sum_{a \in V} W_{a,\alpha}^4 Y_{a,\gamma}^1 \quad (2r_T r_V N_v) \quad (10681)$$

$$\tau_{\gamma,\delta,i}^5 = \sum_{\alpha \in B} \tau_{\delta,\alpha}^3 \tau_{\gamma,\alpha}^4 \tau_{\delta,\alpha,i}^2 \quad (3r_T^2 r_V N_o) \quad (10682)$$

$$\tau_{\gamma,\delta,\epsilon}^6 = \sum_{i \in O} Z_{\gamma,\delta} Y_{i,\delta}^4 \tau_{\gamma,\epsilon,i}^5 \quad (3r_T^3 N_o) \quad (10683)$$

$$\tau_{\gamma,\delta,i}^7 = \sum_{\epsilon \in A} Y_{i,\epsilon}^2 \tau_{\epsilon,\gamma,\delta}^6 \quad (2r_T^3 N_o) \quad (10684)$$

$$\tau_{\gamma,\delta,w}^8 = \sum_{\epsilon \in A} \sum_{i \in O} {}^2D_{i,w}^2 Y_{i,\delta}^{2,*} \tau_{\epsilon,\delta,w}^0 \tau_{\epsilon,\gamma,i}^7 \quad (4r_D r_T^3 N_o) \quad (10685)$$

$$\tau_{\gamma,\delta,w}^9 = \sum_{\epsilon \in A} Z_{\epsilon,\delta}^* \tau_{\gamma,\epsilon,w}^8 \quad (2r_D r_T^3) \quad (10686)$$

$$\tau_{\gamma,\delta,w}^{10} = \sum_{\epsilon \in A} Z_{\gamma,\epsilon} \tau_{\epsilon,\delta,w}^9 \quad (2r_D r_T^3) \quad (10687)$$

$$\tau_{\gamma,\delta,w}^{11} = \sum_{i \in O} {}^2D_{i,w}^4 Y_{i,\gamma}^2 Y_{i,\delta}^{4,*} \quad (3r_D r_T^2 N_o) \quad (10688)$$

$${}^2R_{a,\gamma}^3 \leftarrow \sum_{\delta \in A} \sum_{w \in D} \frac{1}{4} {}^2D_{a,w}^3 Y_{a,\delta}^1 \tau_{\delta,\gamma,w}^{10} \tau_{\delta,\gamma,w}^{11} \quad (4r_D r_T^2 N_v) \quad (10689)$$

Raw expression

$${}^2R_{b,\zeta}^3 \leftarrow \sum_{\gamma \in A} \sum_{i \in O} \sum_{j \in O} \sum_{k \in O} \sum_{l \in O} \sum_{a \in V} \sum_{c \in V} \sum_{d \in V} \frac{1}{4} \quad (10690)$$

$$Y_{a,\gamma}^{1,*} Y_{i,\gamma}^{2,*} Z_{\gamma,\zeta}^* Y_{j,\zeta}^{4,*} {}^2D_{a,i,b,j} {}^2T_{b,k,a,i} {}^2T_{c,l,d,j} V_{k,c,l,d}$$

Factorized expression

$$\tau_{\gamma,\delta,w}^0 = \sum_{i \in O} {}^2D_{i,w}^4 Y_{i,\gamma}^2 Y_{i,\delta}^{4,*} \quad (3r_D r_T^2 N_o) \quad (10691)$$

$$\tau_{\gamma,\delta,w}^1 = \sum_{a \in V} {}^2D_{a,w}^1 Y_{a,\gamma}^3 Y_{a,\delta}^{1,*} \quad (3r_D r_T^2 N_v) \quad (10692)$$

$$\tau_{\gamma,\alpha}^2 = \sum_{a \in V} W_{a,\alpha}^2 Y_{a,\gamma}^3 \quad (2r_T r_V N_v) \quad (10693)$$

$$\tau_{\gamma,\alpha,i}^3 = \sum_{\beta \in B} W_{i,\beta}^1 X_{\beta,\alpha} \tau_{\gamma,\beta}^2 \quad (3r_T r_V^2 N_o) \quad (10694)$$

$$\tau_{\gamma,\alpha}^4 = \sum_{i \in O} W_{i,\alpha}^3 Y_{i,\gamma}^4 \quad (2r_T r_V N_o) \quad (10695)$$

$$\tau_{\gamma,\alpha}^5 = \sum_{a \in V} W_{a,\alpha}^4 Y_{a,\gamma}^1 \quad (2r_T r_V N_v) \quad (10696)$$

$$\tau_{\gamma,\delta,i}^6 = \sum_{\alpha \in B} \tau_{\delta,\alpha}^4 \tau_{\gamma,\alpha}^5 \tau_{\delta,\alpha,i}^3 \quad (3r_T^2 r_V N_o) \quad (10697)$$

$$\tau_{\gamma,i}^7 = \sum_{\delta \in A} Z_{\gamma,\delta} \tau_{\gamma,\delta,i}^6 \quad (2r_T^2 N_o) \quad (10698)$$

$$\tau_{i,j}^8 = \sum_{\gamma \in A} Y_{j,\gamma}^2 \tau_{\gamma,i}^7 \quad (2r_T N_o^2) \quad (10699)$$

$$\tau_{\gamma,i}^9 = \sum_{j \in O} Y_{j,\gamma}^4 \tau_{j,i}^8 \quad (2r_T N_o^2) \quad (10700)$$

$$\tau_{\gamma,\delta,w}^{10} = \sum_{i \in O} {}^2D_{i,w}^2 Y_{i,\gamma}^{2,*} \tau_{i,\delta}^9 \tau_{\gamma,i}^9 \quad (3r_D r_T^2 N_o) \quad (10701)$$

$$\tau_{\gamma,\delta,w}^{11} = \sum_{\epsilon \in A} Z_{\epsilon,\delta}^* \tau_{\gamma,\epsilon,w}^1 \tau_{\gamma,\epsilon,w}^{10} \quad (3r_D r_T^3) \quad (10702)$$

$$\tau_{\gamma,\delta,w}^{12} = \sum_{\epsilon \in A} Z_{\gamma,\epsilon} \tau_{\epsilon,\delta,w}^{11} \quad (2r_D r_T^3) \quad (10703)$$

$${}^2R^3_{a,\gamma} \leftarrow \sum_{\delta \in A} \sum_{w \in D} \frac{1}{4} {}^2D^3_{a,w} Y^1_{a,\delta} \tau^0_{\delta,\gamma,w} \tau^{12}_{\delta,\gamma,w} \quad (4r_D r_T^2 N_v) \quad (10704)$$

$$\tau^{10}_{\gamma,\delta,w} = \sum_{\epsilon \in A} \sum_{i \in O} Y^2_{i,\gamma} Z_{\gamma,\epsilon} \tau^9_{\epsilon,\delta,w,i} \quad (3r_D r_T^3 N_o) \quad (10716)$$

Raw expression

$${}^2R^3_{b,\zeta} \leftarrow \sum_{\gamma \in A} \sum_{i \in O} \sum_{j \in O} \sum_{k \in O} \sum_{l \in O} \sum_{a \in V} \sum_{c \in V} \sum_{d \in V} \frac{1}{4} \quad (10705)$$

$$Y^{1,*}_{a,\gamma} Y^{2,*}_{i,\gamma} Z^*_{\gamma,\zeta} Y^{4,*}_{j,\zeta}$$

$${}^2D^{a,i,b,j} {}^2T_{b,k,a,l} {}^2T_{c,i,d,j} V_{k,d,l,c}$$

Factorized expression

$$\tau^0_{\gamma,\delta,w} = \sum_{a \in V} {}^2D^1_{a,w} Y^3_{a,\gamma} Y^{1,*}_{a,\delta} \quad (3r_D r_T^2 N_v) \quad (10706)$$

$$\tau^1_{\gamma,\delta,w,i} = \sum_{\epsilon \in A} Y^{2,*}_{i,\epsilon} Z^*_{\epsilon,\delta} \tau^0_{\gamma,\epsilon,w} \quad (3r_D r_T^3 N_o) \quad (10707)$$

$$\tau^2_{\gamma,\alpha} = \sum_{a \in V} W^4_{a,\alpha} Y^1_{a,\gamma} \quad (2r_T r_V N_v) \quad (10708)$$

$$\tau^3_{\gamma,\alpha,i} = \sum_{\beta \in B} X_{\alpha,\beta} W^3_{i,\beta} \tau^2_{\gamma,\beta} \quad (3r_T r_V^2 N_o) \quad (10709)$$

$$\tau^4_{\gamma,\alpha} = \sum_{a \in V} W^2_{a,\alpha} Y^3_{a,\gamma} \quad (2r_T r_V N_v) \quad (10710)$$

$$\tau^5_{\gamma,\alpha,i} = \sum_{\delta \in A} Z_{\gamma,\delta} Y^4_{i,\delta} \tau^4_{\delta,\alpha} \quad (3r_T^2 r_V N_o) \quad (10711)$$

$$\tau^6_{\gamma,i,j,k} = \sum_{\alpha \in B} W^1_{i,\alpha} \tau^3_{\gamma,\alpha,j} \tau^5_{\gamma,\alpha,k} \quad (3r_T r_V N_o^3) \quad (10712)$$

$$\tau^7_{i,j,k,l} = \sum_{\gamma \in A} Y^2_{k,\gamma} \tau^6_{\gamma,i,j,l} \quad (2r_T N_o^4) \quad (10713)$$

$$\tau^8_{\gamma,i,j,k} = \sum_{l \in O} Y^4_{l,\gamma} \tau^7_{i,l,j,k} \quad (2r_T N_o^4) \quad (10714)$$

$$\tau^9_{\gamma,\delta,w,i} = \sum_{j \in O} \sum_{k \in O} {}^2D^2_{j,w} {}^2D^4_{k,w} Y^{4,*}_{k,\delta} \tau^1_{\gamma,\delta,w,j} \tau^8_{\gamma,i,j,k} \quad (5r_D r_T^2 N_o^3) \quad (10715)$$

$$\tau^9_{\gamma,\delta,w,i} = \sum_{a \in V} {}^2D^1_{a,w} Y^{1,*}_{a,\delta} \tau^7_{\gamma,a} \quad (3r_D r_T^2 N_v) \quad (10727)$$

$${}^2R^3_{a,\gamma} \leftarrow \sum_{\delta \in A} \sum_{w \in D} \frac{1}{4} {}^2D^3_{a,w} Y^1_{a,\delta} \tau^{10}_{\delta,\gamma,w} \quad (3r_D r_T^2 N_v) \quad (10717)$$

Raw expression

$${}^2R^3_{b,\zeta} \leftarrow \sum_{\gamma \in A} \sum_{i \in O} \sum_{j \in O} \sum_{k \in O} \sum_{l \in O} \sum_{a \in V} \sum_{c \in V} \sum_{d \in V} \frac{1}{4} \quad (10718)$$

$$Y^{1,*}_{a,\gamma} Y^{2,*}_{i,\gamma} Z^*_{\gamma,\zeta} Y^{4,*}_{j,\zeta}$$

$${}^2D^{a,i,b,j} {}^2T_{b,k,a,l} {}^2T_{c,j,d,i} V_{k,c,l,d}$$

Factorized expression

$$\tau^0_{\gamma,\delta,w} = \sum_{i \in O} {}^2D^4_{i,w} Y^2_{i,\gamma} Y^{4,*}_{i,\delta} \quad (3r_D r_T^2 N_o) \quad (10719)$$

$$\tau^1_{\gamma,\alpha} = \sum_{a \in V} W^4_{a,\alpha} Y^1_{a,\gamma} \quad (2r_T r_V N_v) \quad (10720)$$

$$\tau^2_{\gamma,\alpha,i} = \sum_{\beta \in B} X_{\alpha,\beta} W^3_{i,\beta} \tau^1_{\gamma,\beta} \quad (3r_T r_V^2 N_o) \quad (10721)$$

$$\tau^3_{\gamma,\alpha} = \sum_{i \in O} W^1_{i,\alpha} Y^2_{i,\gamma} \quad (2r_T r_V N_o) \quad (10722)$$

$$\tau^4_{\gamma,\alpha} = \sum_{\delta \in A} \sum_{i \in O} Z_{\delta,\gamma} Y^4_{i,\gamma} \tau^3_{\delta,\alpha} \tau^2_{\delta,\alpha,i} \quad (4r_T^2 r_V N_o) \quad (10723)$$

$$\tau^5_{\gamma,a} = \sum_{\alpha \in B} W^2_{a,\alpha} \tau^4_{\gamma,\alpha} \quad (2r_T r_V N_v) \quad (10724)$$

$$\tau^6_{a,b} = \sum_{\gamma \in A} Y^3_{b,\gamma} \tau^5_{\gamma,a} \quad (2r_T N_v^2) \quad (10725)$$

$$\tau^7_{\gamma,a} = \sum_{b \in V} Y^3_{b,\gamma} \tau^6_{b,a} \quad (2r_T N_v^2) \quad (10726)$$

$$\tau^9_{\gamma,\delta,w} = \sum_{i \in O} {}^2D^2_{i,w} Y^4_{i,\gamma} Y^{2,*}_{i,\delta} \quad (3r_D r_T^2 N_o) \quad (10728)$$

$$\tau^{10}_{\gamma,\delta,w} = \sum_{\epsilon \in A} Z^*_{\epsilon,\delta} \tau^8_{\gamma,\epsilon,w} \tau^9_{\gamma,\epsilon,w} \quad (3r_D r_T^3) \quad (10729)$$

$$\tau^{11}_{\gamma,\delta,w} = \sum_{\epsilon \in A} Z_{\gamma,\epsilon} \tau^{10}_{\epsilon,\delta,w} \quad (2r_D r_T^3) \quad (10730)$$

$${}^2R^3_{a,\gamma} \leftarrow \sum_{\delta \in A} \sum_{w \in D} \frac{1}{4} {}^2D^3_{a,w} Y^1_{a,\delta} \tau^0_{\delta,\gamma,w} \tau^{11}_{\delta,\gamma,w} \quad (4r_D r_T^2 N_v) \quad (10731)$$

Raw expression

$${}^2R^3_{b,\zeta} \leftarrow \sum_{\gamma \in A} \sum_{i \in O} \sum_{j \in O} \sum_{k \in O} \sum_{l \in O} \sum_{a \in V} \sum_{c \in V} \sum_{d \in V} \frac{1}{4} \quad (10732)$$

$$Y^{1,*}_{a,\gamma} \quad Y^{2,*}_{i,\gamma} \quad Z^*_{\gamma,\zeta} \quad Y^{4,*}_{j,\zeta} \quad {}^2D^{a,i,b,j} \quad {}^2T_{b,k,c,i} \quad {}^2T_{d,j,a,l} \quad V_{l,c,k,d}$$

Factorized expression

$$\tau^0_{\gamma,\delta,w} = \sum_{i \in O} {}^2D^4_{i,w} Y^2_{i,\gamma} Y^{4,*}_{i,\delta} \quad (3r_D r_T^2 N_o) \quad (10733)$$

$$\tau^1_{\gamma,\delta,w} = \sum_{a \in V} {}^2D^1_{a,w} Y^3_{a,\gamma} Y^{1,*}_{a,\delta} \quad (3r_D r_T^2 N_v) \quad (10734)$$

$$\tau^2_{\gamma,\delta,w} = \sum_{i \in O} {}^2D^2_{i,w} Y^4_{i,\gamma} Y^{2,*}_{i,\delta} \quad (3r_D r_T^2 N_o) \quad (10735)$$

$$\tau^3_{\gamma,\delta,w} = \sum_{\epsilon \in A} Z^*_{\epsilon,\delta} \tau^1_{\gamma,\epsilon,w} \tau^2_{\gamma,\epsilon,w} \quad (3r_D r_T^3) \quad (10736)$$

$$\tau^4_{\gamma,\delta,w} = \sum_{\epsilon \in A} Z_{\gamma,\epsilon} \tau^3_{\epsilon,\delta,w} \quad (2r_D r_T^3) \quad (10737)$$

$$\tau^5_{\gamma,\alpha} = \sum_{a \in V} W^2_{a,\alpha} Y^3_{a,\gamma} \quad (2r_T r_V N_v) \quad (10738)$$

$$\tau^6_{\gamma,\alpha,i} = \sum_{\beta \in B} W^1_{i,\beta} X_{\beta,\alpha} \tau^5_{\gamma,\beta} \quad (3r_T r_V^2 N_o) \quad (10739)$$

$$\tau^7_{\gamma,\alpha} = \sum_{i \in O} W^3_{i,\alpha} Y^4_{i,\gamma} \quad (2r_T r_V N_o) \quad (10740)$$

$$\tau^8_{\gamma,\alpha} = \sum_{\delta \in A} \sum_{i \in O} Y^2_{i,\gamma} Z_{\gamma,\delta} \tau^7_{\delta,\alpha} \tau^6_{\delta,\alpha,i} \quad (4r_T^2 r_V N_o) \quad (10741)$$

$$\tau^9_{\gamma,a} = \sum_{\alpha \in B} W^4_{a,\alpha} \tau^8_{\gamma,\alpha} \quad (2r_T r_V N_v) \quad (10742)$$

$$\tau^{10}_{\gamma,\delta} = \sum_{a \in V} Y^1_{a,\gamma} \tau^9_{\delta,a} \quad (2r_T^2 N_v) \quad (10743)$$

$$\tau^{11}_{\gamma,a} = \sum_{\delta \in A} Y^1_{a,\delta} \tau^{10}_{\gamma,\delta} \quad (2r_T^2 N_v) \quad (10744)$$

$${}^2R^3_{a,\gamma} \leftarrow \sum_{\delta \in A} \sum_{w \in D} \frac{1}{4} {}^2D^3_{a,w} \tau^{11}_{\delta,a} \tau^0_{\delta,\gamma,w} \tau^4_{\delta,\gamma,w} \quad (4r_D r_T^2 N_v) \quad (10745)$$

Raw expression

$${}^2R^3_{b,\zeta} \leftarrow \sum_{\gamma \in A} \sum_{i \in O} \sum_{j \in O} \sum_{k \in O} \sum_{l \in O} \sum_{a \in V} \sum_{c \in V} \sum_{d \in V} \frac{1}{4} \quad (10746)$$

$$Y^{1,*}_{a,\gamma} \quad Y^{2,*}_{i,\gamma} \quad Z^*_{\gamma,\zeta} \quad Y^{4,*}_{j,\zeta} \quad {}^2D^{a,i,b,j} \quad {}^2T_{b,k,c,j} \quad {}^2T_{d,i,a,l} \quad V_{l,d,k,c}$$

Factorized expression

$$\tau^0_{\gamma,\alpha} = \sum_{a \in V} W^2_{a,\alpha} Y^3_{a,\gamma} \quad (2r_T r_V N_v) \quad (10747)$$

$$\tau^1_{\gamma,\alpha,i} = \sum_{\beta \in B} W^1_{i,\beta} X_{\beta,\alpha} \tau^0_{\gamma,\beta} \quad (3r_T r_V^2 N_o) \quad (10748)$$

$$\tau^2_{\gamma,\alpha} = \sum_{i \in O} W^3_{i,\alpha} Y^4_{i,\gamma} \quad (2r_T r_V N_o) \quad (10749)$$

$$\tau^3_{\gamma,\alpha} = \sum_{a \in V} W^4_{a,\alpha} Y^1_{a,\gamma} \quad (2r_T r_V N_v) \quad (10750)$$

$$\tau^4_{\gamma,\delta,i} = \sum_{\alpha \in B} \tau^2_{\delta,\alpha} \tau^3_{\gamma,\alpha} \tau^1_{\delta,\alpha,i} \quad (3r_T^2 r_V N_o) \quad (10751)$$

$$\tau^5_{\gamma,i} = \sum_{\delta \in A} Z_{\gamma,\delta} \tau^4_{\gamma,\delta,i} \quad (2r_T^2 N_o) \quad (10752)$$

$$\tau^6_{i,j} = \sum_{\gamma \in A} Y^2_{j,\gamma} \tau^5_{\gamma,i} \quad (2r_T N_o^2) \quad (10753)$$

$$\tau^7_{\gamma,i} = \sum_{j \in O} Y^2_{j,\gamma} \tau^6_{j,i} \quad (2r_T N_o^2) \quad (10754)$$

$$\tau^5_{\gamma,\delta,\alpha,w} = \sum_{i \in O} {}^2D^4_{i,w} Y^{4,*}_{i,\delta} \tau^4_{\gamma,\alpha,i} \quad (3r_D r_T^2 r_V N_o) \quad (10767)$$

$$\tau^8_{\gamma,\delta,w} = \sum_{i \in O} {}^2D^4_{i,w} Y^{4,*}_{i,\delta} \tau^7_{\gamma,i} \quad (3r_D r_T^2 N_o) \quad (10755)$$

$$\tau^6_{\gamma,\delta,w} = \sum_{a \in V} {}^2D^1_{a,w} Y^3_{a,\gamma} Y^{1,*}_{a,\delta} \quad (3r_D r_T^2 N_v) \quad (10768)$$

$$\tau^9_{\gamma,\delta,w} = \sum_{a \in V} {}^2D^1_{a,w} Y^3_{a,\gamma} Y^{1,*}_{a,\delta} \quad (3r_D r_T^2 N_v) \quad (10756)$$

$$\tau^7_{\gamma,\delta,w,i} = \sum_{\epsilon \in A} Y^{2,*}_{i,\epsilon} Z^*_{\epsilon,\delta} \tau^6_{\gamma,\epsilon,w} \quad (3r_D r_T^3 N_o) \quad (10769)$$

$$\tau^{10}_{\gamma,\delta,w} = \sum_{i \in O} {}^2D^2_{i,w} Y^4_{i,\gamma} Y^{2,*}_{i,\delta} \quad (3r_D r_T^2 N_o) \quad (10757)$$

$$\tau^8_{\gamma,\delta,\epsilon,w} = \sum_{i \in O} {}^2D^2_{i,w} Y^4_{i,\delta} \tau^7_{\gamma,\epsilon,w,i} \quad (3r_D r_T^3 N_o) \quad (10770)$$

$$\tau^{11}_{\gamma,\delta,w} = \sum_{\epsilon \in A} Z^*_{\epsilon,\delta} \tau^{10}_{\gamma,\epsilon,w} \tau^9_{\gamma,\epsilon,w} \quad (3r_D r_T^3) \quad (10758)$$

$$\tau^9_{\gamma,\delta,\alpha,w} = \sum_{\epsilon \in A} \tau^2_{\gamma,\epsilon,\alpha} \tau^5_{\epsilon,\delta,\alpha,w} \tau^8_{\epsilon,\gamma,\delta,w} \quad (3r_D r_T^3 r_V) \quad (10771)$$

$$\tau^{12}_{\gamma,\delta,w} = \sum_{\epsilon \in A} Z_{\gamma,\epsilon} \tau^{11}_{\epsilon,\delta,w} \quad (2r_D r_T^3) \quad (10759)$$

$${}^2R^3_{a,\gamma} \leftarrow \sum_{\delta \in A} \sum_{w \in D} \frac{1}{4} {}^2D^3_{a,w} Y^1_{a,\delta} \tau^{12}_{\delta,\gamma,w} \tau^8_{\delta,\gamma,w} \quad (4r_D r_T^2 N_v) \quad (10760)$$

$$\tau^{10}_{\gamma,\delta,w,i} = \sum_{\alpha \in B} W^3_{i,\alpha} \tau^9_{\gamma,\delta,\alpha,w} \quad (2r_D r_T^2 r_V N_o) \quad (10772)$$

Raw expression

$${}^2R^3_{b,\zeta} \leftarrow \sum_{\gamma \in A} \sum_{i \in O} \sum_{j \in O} \sum_{k \in O} \sum_{l \in O} \sum_{a \in V} \sum_{c \in V} \sum_{d \in V} \frac{1}{4} \quad (10761)$$

$$Y^{1,*}_{a,\gamma} Y^{2,*}_{i,\gamma} Z^*_{\gamma,\zeta} Y^{4,*}_{j,\zeta} {}^2D^{a,i,b,j} {}^2T_{b,k,c,j} {}^2T_{d,l,a,i} V_{l,c,k,d}$$

$$\tau^{11}_{\gamma,\delta,w} = \sum_{\epsilon \in A} \sum_{i \in O} Y^2_{i,\gamma} Z_{\gamma,\epsilon} \tau^{10}_{\epsilon,\delta,w,i} \quad (3r_D r_T^3 N_o) \quad (10773)$$

$${}^2R^3_{a,\gamma} \leftarrow \sum_{\delta \in A} \sum_{w \in D} \frac{1}{4} {}^2D^3_{a,w} Y^1_{a,\delta} \tau^{11}_{\delta,\gamma,w} \quad (3r_D r_T^2 N_v) \quad (10774)$$

Factorized expression

$$\tau^0_{\gamma,\alpha} = \sum_{a \in V} W^2_{a,\alpha} Y^3_{a,\gamma} \quad (2r_T r_V N_v) \quad (10762)$$

Raw expression

$$\tau^1_{\gamma,\alpha,i} = \sum_{\beta \in B} W^1_{i,\beta} X_{\beta,\alpha} \tau^0_{\gamma,\beta} \quad (3r_T r_V^2 N_o) \quad (10763)$$

$${}^2R^3_{b,\zeta} \leftarrow \sum_{\gamma \in A} \sum_{i \in O} \sum_{j \in O} \sum_{k \in O} \sum_{l \in O} \sum_{a \in V} \sum_{c \in V} \sum_{d \in V} \frac{1}{4} \quad (10775)$$

$$Y^{1,*}_{a,\gamma} Y^{2,*}_{i,\gamma} Z^*_{\gamma,\zeta} Y^{4,*}_{j,\zeta} {}^2D^{a,i,b,j} {}^2T_{b,k,c,l} {}^2T_{d,j,a,i} V_{k,c,l,d}$$

$$\tau^2_{\gamma,\delta,\alpha} = \sum_{i \in O} Y^4_{i,\delta} \tau^1_{\gamma,\alpha,i} \quad (2r_T^2 r_V N_o) \quad (10764)$$

Factorized expression

$$\tau^3_{\gamma,\alpha} = \sum_{a \in V} W^4_{a,\alpha} Y^1_{a,\gamma} \quad (2r_T r_V N_v) \quad (10765)$$

$$\tau^0_{\gamma,\delta,w} = \sum_{a \in V} {}^2D^1_{a,w} Y^3_{a,\gamma} Y^{1,*}_{a,\delta} \quad (3r_D r_T^2 N_v) \quad (10776)$$

$$\tau^4_{\gamma,\alpha,i} = \sum_{\delta \in A} Y^2_{i,\delta} Z_{\delta,\gamma} \tau^3_{\delta,\alpha} \quad (3r_T^2 r_V N_o) \quad (10766)$$

$$\tau^1_{\gamma,\delta,w} = \sum_{i \in O} {}^2D^2_{i,w} Y^4_{i,\gamma} Y^{2,*}_{i,\delta} \quad (3r_D r_T^2 N_o) \quad (10777)$$

$$\tau_{\gamma,\delta,w}^2 = \sum_{\epsilon \in A} Z_{\epsilon,\delta}^* \tau_{\gamma,\epsilon,w}^0 \tau_{\gamma,\epsilon,w}^1 \quad (3r_D r_T^3) \quad (10778)$$

$$\tau_{\gamma,\alpha,i}^1 = \sum_{\beta \in B} W_{i,\beta}^1 X_{\beta,\alpha} \tau_{\gamma,\beta}^0 \quad (3r_T r_V^2 N_o) \quad (10791)$$

$$\tau_{\gamma,\delta,w}^3 = \sum_{\epsilon \in A} Z_{\gamma,\epsilon} \tau_{\epsilon,\delta,w}^2 \quad (2r_D r_T^3) \quad (10779)$$

$$\tau_{\gamma,\delta,\alpha}^2 = \sum_{i \in O} Y_{i,\delta}^4 \tau_{\gamma,\alpha,i}^1 \quad (2r_T^2 r_V N_o) \quad (10792)$$

$$\tau_{\gamma,\alpha}^4 = \sum_{a \in V} W_{a,\alpha}^4 Y_{a,\gamma}^1 \quad (2r_T r_V N_v) \quad (10780)$$

$$\tau_{\gamma,\alpha}^3 = \sum_{a \in V} W_{a,\alpha}^4 Y_{a,\gamma}^1 \quad (2r_T r_V N_v) \quad (10793)$$

$$\tau_{\gamma,\alpha,i}^5 = \sum_{\beta \in B} X_{\alpha,\beta} W_{i,\beta}^3 \tau_{\gamma,\beta}^4 \quad (3r_T r_V^2 N_o) \quad (10781)$$

$$\tau_{\gamma,\alpha,i}^4 = \sum_{\delta \in A} Y_{i,\delta}^2 Z_{\delta,\gamma} \tau_{\delta,\alpha}^3 \quad (3r_T^2 r_V N_o) \quad (10794)$$

$$\tau_{\gamma,\alpha}^6 = \sum_{i \in O} W_{i,\alpha}^1 Y_{i,\gamma}^2 \quad (2r_T r_V N_o) \quad (10782)$$

$$\tau_{\gamma,\delta,\alpha,w}^5 = \sum_{i \in O} {}^2D_{i,w}^4 Y_{i,\delta}^{4,*} \tau_{\gamma,\alpha,i}^4 \quad (3r_D r_T^2 r_V N_o) \quad (10795)$$

$$\tau_{\gamma,\alpha}^7 = \sum_{a \in V} W_{a,\alpha}^2 Y_{a,\gamma}^3 \quad (2r_T r_V N_v) \quad (10783)$$

$$\tau_{\gamma,\delta,w}^6 = \sum_{a \in V} {}^2D_{a,w}^1 Y_{a,\gamma}^3 Y_{a,\delta}^{1,*} \quad (3r_D r_T^2 N_v) \quad (10796)$$

$$\tau_{\gamma,\delta,i}^8 = \sum_{\alpha \in B} \tau_{\gamma,\alpha}^6 \tau_{\delta,\alpha}^7 \tau_{\gamma,\alpha,i}^5 \quad (3r_T^2 r_V N_o) \quad (10784)$$

$$\tau_{\gamma,\delta,w,i}^7 = \sum_{\epsilon \in A} Y_{i,\epsilon}^{2,*} Z_{\epsilon,\delta}^* \tau_{\gamma,\epsilon,w}^6 \quad (3r_D r_T^3 N_o) \quad (10797)$$

$$\tau_{\gamma,\delta,i}^{10} = \sum_{\epsilon \in A} Y_{i,\epsilon}^4 \tau_{\gamma,\delta,\epsilon}^9 \quad (2r_T^3 N_o) \quad (10786)$$

$$\tau_{\gamma,\delta,\epsilon,w}^8 = \sum_{i \in O} {}^2D_{i,w}^2 Y_{i,\gamma}^2 \tau_{\delta,\epsilon,w,i}^7 \quad (3r_D r_T^3 N_o) \quad (10798)$$

$$\tau_{\gamma,\delta,w}^{11} = \sum_{\epsilon \in A} \sum_{i \in O} {}^2D_{i,w}^4 Y_{i,\delta}^{4,*} \tau_{\epsilon,\gamma,i}^{10} \tau_{\epsilon,\delta,w}^3 \quad (4r_D r_T^3 N_o) \quad (10787)$$

$$\tau_{\gamma,\delta,\alpha,w}^9 = \sum_{\epsilon \in A} \tau_{\gamma,\epsilon,\alpha}^2 \tau_{\epsilon,\delta,\alpha,w}^5 \tau_{\gamma,\epsilon,\delta,w}^8 \quad (3r_D r_T^3 r_V) \quad (10799)$$

$${}^2R_{a,\gamma}^3 \leftarrow \sum_{\delta \in A} \sum_{w \in D} \frac{1}{4} {}^2D_{a,w}^3 Y_{a,\delta}^1 \tau_{\delta,\gamma,w}^{11} \quad (3r_D r_T^2 N_v) \quad (10788)$$

$$\tau_{\gamma,\delta,w,i}^{10} = \sum_{\alpha \in B} W_{i,\alpha}^3 \tau_{\gamma,\delta,\alpha,w}^9 \quad (2r_D r_T^2 r_V N_o) \quad (10800)$$

Raw expression

$${}^2R_{b,\zeta}^3 \leftarrow \sum_{\gamma \in A} \sum_{i \in O} \sum_{j \in O} \sum_{k \in O} \sum_{l \in O} \sum_{a \in V} \sum_{c \in V} \sum_{d \in V} \frac{1}{4} \quad (10789)$$

$$Y_{a,\gamma}^{1,*} Y_{i,\gamma}^{2,*} Z_{\gamma,\zeta}^* Y_{j,\zeta}^{4,*} {}^2D_{a,i,b,j} {}^2T_{c,i,b,j} {}^2T_{d,k,a,l} V_{k,c,l,d}$$

$$\tau_{\gamma,\delta,w}^{11} = \sum_{\epsilon \in A} \sum_{i \in O} Z_{\epsilon,\gamma} Y_{i,\gamma}^4 \tau_{\epsilon,\delta,w,i}^{10} \quad (3r_D r_T^3 N_o) \quad (10801)$$

Factorized expression

$${}^2R_{a,\gamma}^3 \leftarrow \sum_{\delta \in A} \sum_{w \in D} \frac{1}{4} {}^2D_{a,w}^3 Y_{a,\delta}^3 \tau_{\delta,\gamma,w}^{11} \quad (3r_D r_T^2 N_v) \quad (10802)$$

Raw expression

$$\tau_{\gamma,\alpha}^0 = \sum_{a \in V} W_{a,\alpha}^2 Y_{a,\gamma}^1 \quad (2r_T r_V N_v) \quad (10790)$$



$${}^2R^3_{b,\zeta} \leftarrow \sum_{\gamma \in A} \sum_{i \in O} \sum_{j \in O} \sum_{k \in O} \sum_{l \in O} \sum_{a \in V} \sum_{c \in V} \sum_{d \in V} \frac{1}{4} \quad (10803)$$

$$Y^{1,*}_{a,\gamma} \ Y^{2,*}_{i,\gamma} \ Z^*_{\gamma,\zeta} \ Y^{4,*}_{j,\zeta}$$

$${}^2D^{a,i,b,j} \ {}^2T_{c,i,b,k} \ {}^2T_{d,j,a,l} \ V_{l,c,k,d}$$

Factorized expression

$$\tau^0_{\gamma,\delta,w} = \sum_{i \in O} {}^2D^4_{i,w} Y^4_{i,\gamma} Y^{4,*}_{i,\delta} \quad (3r_D r_T^2 N_o) \quad (10804)$$

$$\tau^1_{\gamma,\delta,w} = \sum_{i \in O} {}^2D^2_{i,w} Y^2_{i,\gamma} Y^{2,*}_{i,\delta} \quad (3r_D r_T^2 N_o) \quad (10805)$$

$$\tau^2_{\gamma,\alpha} = \sum_{a \in V} W^4_{a,\alpha} Y^1_{a,\gamma} \quad (2r_T r_V N_v) \quad (10806)$$

$$\tau^3_{\gamma,\alpha,i} = \sum_{\beta \in B} X_{\alpha,\beta} W^3_{i,\beta} \tau^2_{\gamma,\beta} \quad (3r_T r_V^2 N_o) \quad (10807)$$

$$\tau^4_{\gamma,\alpha} = \sum_{i \in O} W^1_{i,\alpha} Y^2_{i,\gamma} \quad (2r_T r_V N_o) \quad (10808)$$

$$\tau^5_{\gamma,\alpha} = \sum_{\delta \in A} \sum_{i \in O} Z_{\delta,\gamma} Y^4_{i,\gamma} \tau^4_{\delta,\alpha} \tau^3_{\delta,\alpha,i} \quad (4r_T^2 r_V N_o) \quad (10809)$$

$$\tau^6_{\gamma,a} = \sum_{\alpha \in B} W^2_{a,\alpha} \tau^5_{\gamma,\alpha} \quad (2r_T r_V N_v) \quad (10810)$$

$$\tau^7_{a,b} = \sum_{\gamma \in A} Y^3_{b,\gamma} \tau^6_{\gamma,a} \quad (2r_T N_v^2) \quad (10811)$$

$$\tau^8_{\gamma,a} = \sum_{b \in V} Y^1_{b,\gamma} \tau^7_{b,a} \quad (2r_T N_v^2) \quad (10812)$$

$$\tau^9_{\gamma,\delta,w} = \sum_{a \in V} {}^2D^1_{a,w} Y^{1,*}_{a,\delta} \tau^8_{\gamma,a} \quad (3r_D r_T^2 N_v) \quad (10813)$$

$$\tau^{10}_{\gamma,\delta,w} = \sum_{\epsilon \in A} Z^*_{\epsilon,\delta} \tau^1_{\gamma,\epsilon,w} \tau^9_{\gamma,\epsilon,w} \quad (3r_D r_T^3) \quad (10814)$$

$$\tau^{11}_{\gamma,\delta,w} = \sum_{\epsilon \in A} Z_{\epsilon,\gamma} \tau^{10}_{\epsilon,\delta,w} \quad (2r_D r_T^3) \quad (10815)$$

$${}^2R^3_{a,\gamma} \leftarrow \sum_{\delta \in A} \sum_{w \in D} \frac{1}{4} {}^2D^3_{a,w} Y^3_{a,\delta} \tau^0_{\delta,\gamma,w} \tau^{11}_{\delta,\gamma,w} \quad (4r_D r_T^2 N_v) \quad (10816)$$

Raw expression

$${}^2R^3_{b,\zeta} \leftarrow \sum_{\gamma \in A} \sum_{i \in O} \sum_{j \in O} \sum_{k \in O} \sum_{l \in O} \sum_{a \in V} \sum_{c \in V} \sum_{d \in V} \frac{1}{4} \quad (10817)$$

$$Y^{1,*}_{a,\gamma} \ Y^{2,*}_{i,\gamma} \ Z^*_{\gamma,\zeta} \ Y^{4,*}_{j,\zeta}$$

$${}^2D^{a,i,b,j} \ {}^2T_{c,j,b,k} \ {}^2T_{d,i,a,l} \ V_{l,d,k,c}$$

Factorized expression

$$\tau^0_{\gamma,\delta,w} = \sum_{i \in O} {}^2D^4_{i,w} Y^2_{i,\gamma} Y^{4,*}_{i,\delta} \quad (3r_D r_T^2 N_o) \quad (10818)$$

$$\tau^1_{\gamma,\delta,w} = \sum_{a \in V} {}^2D^1_{a,w} Y^3_{a,\gamma} Y^{1,*}_{a,\delta} \quad (3r_D r_T^2 N_v) \quad (10819)$$

$$\tau^2_{\gamma,\delta,w} = \sum_{i \in O} {}^2D^2_{i,w} Y^4_{i,\gamma} Y^{2,*}_{i,\delta} \quad (3r_D r_T^2 N_o) \quad (10820)$$

$$\tau^3_{\gamma,\delta,w} = \sum_{\epsilon \in A} Z^*_{\epsilon,\delta} \tau^1_{\gamma,\epsilon,w} \tau^2_{\gamma,\epsilon,w} \quad (3r_D r_T^3) \quad (10821)$$

$$\tau^4_{\gamma,\delta,w} = \sum_{\epsilon \in A} Z_{\gamma,\epsilon} \tau^3_{\epsilon,\delta,w} \quad (2r_D r_T^3) \quad (10822)$$

$$\tau^5_{\gamma,\alpha} = \sum_{a \in V} W^4_{a,\alpha} Y^1_{a,\gamma} \quad (2r_T r_V N_v) \quad (10823)$$

$$\tau^6_{\gamma,\alpha,i} = \sum_{\beta \in B} X_{\alpha,\beta} W^3_{i,\beta} \tau^5_{\gamma,\beta} \quad (3r_T r_V^2 N_o) \quad (10824)$$

$$\tau^7_{\gamma,\alpha} = \sum_{i \in O} W^1_{i,\alpha} Y^2_{i,\gamma} \quad (2r_T r_V N_o) \quad (10825)$$

$$\tau^8_{\gamma,\alpha} = \sum_{\delta \in A} \sum_{i \in O} Z_{\delta,\gamma} Y^4_{i,\gamma} \tau^7_{\delta,\alpha} \tau^6_{\delta,\alpha,i} \quad (4r_T^2 r_V N_o) \quad (10826)$$

$$\tau^9_{\gamma,a} = \sum_{\alpha \in B} W^2_{a,\alpha} \tau^8_{\gamma,\alpha} \quad (2r_T r_V N_v) \quad (10827)$$

$$\tau^{10}_{a,b} = \sum_{\gamma \in A} Y^3_{b,\gamma} \tau^9_{\gamma,a} \quad (2r_T N_v^2) \quad (10828)$$

$$\tau^{11}_{\gamma,a} = \sum_{b \in V} Y^1_{b,\gamma} \tau^{10}_{b,a} \quad (2r_T N_v^2) \quad (10829)$$

$$\tau^{10}_{\gamma,\delta,i} = \sum_{\epsilon \in A} Y^2_{i,\epsilon} \tau^9_{\gamma,\epsilon,\delta} \quad (2r_T^3 N_o) \quad (10842)$$

$${}^2R^3_{a,\gamma} \leftarrow \sum_{\delta \in A} \sum_{w \in D} \frac{1}{4} {}^2D^3_{a,w} \tau^{11}_{\delta,a} \tau^0_{\delta,\gamma,w} \tau^4_{\delta,\gamma,w} \quad (4r_D r_T^2 N_v) \tau^{11}_{\gamma,\delta,w} = \sum_{\epsilon \in A} \sum_{i \in O} {}^2D^4_{i,w} Y^{4,*}_{i,\delta} \tau^{10}_{\epsilon,\gamma,i} \tau^3_{\epsilon,\delta,w} \quad (4r_D r_T^3 N_o) \quad (10830) \quad (10843)$$

Raw expression

$${}^2R^3_{b,\zeta} \leftarrow \sum_{\gamma \in A} \sum_{i \in O} \sum_{j \in O} \sum_{k \in O} \sum_{l \in O} \sum_{a \in V} \sum_{c \in V} \sum_{d \in V} \frac{1}{4} \quad (10831)$$

$$Y^{1,*}_{a,\gamma} \quad Y^{2,*}_{i,\gamma} \quad Z^*_{\gamma,\zeta} \quad Y^{4,*}_{j,\zeta}$$

$${}^2D^{a,i,b,j} \quad {}^2T_{c,j,b,k} \quad {}^2T_{d,l,a,i} \quad V_{l,c,k,d}$$

Factorized expression

$$\tau^0_{\gamma,\delta,w} = \sum_{a \in V} {}^2D^1_{a,w} Y^3_{a,\gamma} Y^{1,*}_{a,\delta} \quad (3r_D r_T^2 N_v) \quad (10832)$$

$$\tau^1_{\gamma,\delta,w} = \sum_{i \in O} {}^2D^2_{i,w} Y^4_{i,\gamma} Y^{2,*}_{i,\delta} \quad (3r_D r_T^2 N_o) \quad (10833)$$

$$\tau^2_{\gamma,\delta,w} = \sum_{\epsilon \in A} Z^*_{\epsilon,\delta} \tau^0_{\gamma,\epsilon,w} \tau^1_{\gamma,\epsilon,w} \quad (3r_D r_T^3) \quad (10834)$$

$$\tau^3_{\gamma,\delta,w} = \sum_{\epsilon \in A} Z_{\gamma,\epsilon} \tau^2_{\epsilon,\delta,w} \quad (2r_D r_T^3) \quad (10835)$$

$$\tau^4_{\gamma,\alpha} = \sum_{a \in V} W^4_{a,\alpha} Y^1_{a,\gamma} \quad (2r_T r_V N_v) \quad (10836)$$

$$\tau^5_{\gamma,\alpha,i} = \sum_{\beta \in B} X_{\alpha,\beta} W^3_{i,\beta} \tau^4_{\gamma,\beta} \quad (3r_T r_V^2 N_o) \quad (10837)$$

$$\tau^6_{\gamma,\alpha} = \sum_{i \in O} W^1_{i,\alpha} Y^2_{i,\gamma} \quad (2r_T r_V N_o) \quad (10838)$$

$$\tau^7_{\gamma,\alpha} = \sum_{a \in V} W^2_{a,\alpha} Y^1_{a,\gamma} \quad (2r_T r_V N_v) \quad (10839)$$

$$\tau^8_{\gamma,\delta,i} = \sum_{\alpha \in B} \tau^6_{\gamma,\alpha} \tau^7_{\delta,\alpha} \tau^5_{\gamma,\alpha,i} \quad (3r_T^2 r_V N_o) \quad (10840)$$

$$\tau^9_{\gamma,\delta,\epsilon} = \sum_{i \in O} Z_{\delta,\epsilon} Y^4_{i,\epsilon} \tau^8_{\gamma,\delta,i} \quad (3r_T^3 N_o) \quad (10841)$$

$${}^2R^3_{a,\gamma} \leftarrow \sum_{\delta \in A} \sum_{w \in D} \frac{1}{4} {}^2D^3_{a,w} Y^3_{a,\delta} \tau^{11}_{\delta,\gamma,w} \quad (3r_D r_T^2 N_v) \quad (10844)$$

Raw expression

$${}^2R^3_{b,\zeta} \leftarrow \sum_{\gamma \in A} \sum_{i \in O} \sum_{j \in O} \sum_{k \in O} \sum_{l \in O} \sum_{a \in V} \sum_{c \in V} \sum_{d \in V} \frac{1}{4} \quad (10845)$$

$$Y^{1,*}_{a,\gamma} \quad Y^{2,*}_{i,\gamma} \quad Z^*_{\gamma,\zeta} \quad Y^{4,*}_{j,\zeta}$$

$${}^2D^{a,i,b,j} \quad {}^2T_{c,k,b,j} \quad {}^2T_{d,i,a,l} \quad V_{l,c,k,d}$$

Factorized expression

$$\tau^0_{\gamma,\delta,w} = \sum_{a \in V} {}^2D^1_{a,w} Y^3_{a,\gamma} Y^{1,*}_{a,\delta} \quad (3r_D r_T^2 N_v) \quad (10846)$$

$$\tau^1_{\gamma,\alpha} = \sum_{a \in V} W^2_{a,\alpha} Y^1_{a,\gamma} \quad (2r_T r_V N_v) \quad (10847)$$

$$\tau^2_{\gamma,\alpha,i} = \sum_{\beta \in B} W^1_{i,\beta} X_{\beta,\alpha} \tau^1_{\gamma,\beta} \quad (3r_T r_V^2 N_o) \quad (10848)$$

$$\tau^3_{\gamma,\alpha} = \sum_{i \in O} W^3_{i,\alpha} Y^2_{i,\gamma} \quad (2r_T r_V N_o) \quad (10849)$$

$$\tau^4_{\gamma,\alpha} = \sum_{a \in V} W^4_{a,\alpha} Y^1_{a,\gamma} \quad (2r_T r_V N_v) \quad (10850)$$

$$\tau^5_{\gamma,\delta,i} = \sum_{\alpha \in B} \tau^3_{\gamma,\alpha} \tau^4_{\delta,\alpha} \tau^2_{\gamma,\alpha,i} \quad (3r_T^2 r_V N_o) \quad (10851)$$

$$\tau^6_{\gamma,\delta,\epsilon} = \sum_{i \in O} Z_{\delta,\epsilon} Y^4_{i,\epsilon} \tau^5_{\gamma,\delta,i} \quad (3r_T^3 N_o) \quad (10852)$$

$$\tau^7_{\gamma,\delta,i} = \sum_{\epsilon \in A} Y^2_{i,\epsilon} \tau^6_{\gamma,\epsilon,\delta} \quad (2r_T^3 N_o) \quad (10853)$$

$$\tau_{\gamma,\delta,w}^8 = \sum_{\epsilon \in A} \sum_{i \in O} {}^2D_{i,w}^2 Y_{i,\delta}^{2,*} \tau_{\epsilon,\delta,w}^0 \tau_{\gamma,\epsilon,i}^7 \quad (4r_D r_T^3 N_o) \quad (10854)$$

$$\tau_{\gamma,\delta,w}^9 = \sum_{\epsilon \in A} Z_{\epsilon,\delta}^* \tau_{\gamma,\epsilon,w}^8 \quad (2r_D r_T^3) \quad (10855)$$

$$\tau_{\gamma,\delta,w}^{10} = \sum_{\epsilon \in A} Z_{\epsilon,\gamma} \tau_{\epsilon,\delta,w}^9 \quad (2r_D r_T^3) \quad (10856)$$

$$\tau_{\gamma,\delta,w}^{11} = \sum_{i \in O} {}^2D_{i,w}^4 Y_{i,\gamma}^4 Y_{i,\delta}^{4,*} \quad (3r_D r_T^2 N_o) \quad (10857)$$

$${}^2R_{a,\gamma}^3 \leftarrow \sum_{\delta \in A} \sum_{w \in D} \frac{1}{4} {}^2D_{a,w}^3 Y_{a,\delta}^3 \tau_{\delta,\gamma,w}^{10} \tau_{\delta,\gamma,w}^{11} \quad (4r_D r_T^2 N_v) \quad (10858)$$

Raw expression

$${}^2R_{b,\zeta}^3 \leftarrow \sum_{\gamma \in A} \sum_{i \in O} \sum_{j \in O} \sum_{k \in O} \sum_{l \in O} \sum_{a \in V} \sum_{c \in V} \sum_{d \in V} \frac{1}{4} \quad (10859)$$

$$Y_{a,\gamma}^{1,*} Y_{i,\gamma}^{2,*} Z_{\gamma,\zeta}^* Y_{j,\zeta}^{4,*} {}^2D_{a,i,b,j} {}^2T_{c,k,b,l} {}^2T_{d,j,a,i} V_{k,d,l,c}$$

Factorized expression

$$\tau_{\gamma,\delta,w}^0 = \sum_{a \in V} {}^2D_{a,w}^1 Y_{a,\gamma}^3 Y_{a,\delta}^{1,*} \quad (3r_D r_T^2 N_v) \quad (10860)$$

$$\tau_{\gamma,\alpha}^1 = \sum_{a \in V} W_{a,\alpha}^2 Y_{a,\gamma}^1 \quad (2r_T r_V N_v) \quad (10861)$$

$$\tau_{\gamma,\alpha,i}^2 = \sum_{\delta \in A} Y_{i,\delta}^2 Z_{\delta,\gamma} \tau_{\delta,\alpha}^1 \quad (3r_T^2 r_V N_o) \quad (10862)$$

$$\tau_{\gamma,\alpha}^3 = \sum_{i \in O} W_{i,\alpha}^1 Y_{i,\gamma}^4 \quad (2r_T r_V N_o) \quad (10863)$$

$$\tau_{\gamma,\alpha,w}^4 = \sum_{\delta \in A} \sum_{i \in O} {}^2D_{i,w}^2 Y_{i,\delta}^{2,*} \tau_{i,\gamma}^3 \tau_{\delta,\alpha}^0 \tau_{\delta,\gamma,w}^0 \tau_{\delta,\alpha,i}^2 \quad (5r_D r_T^2 r_V N_o) \quad (10864)$$

$$\tau_{\gamma,\alpha,w}^5 = \sum_{\beta \in B} X_{\beta,\alpha} \tau_{\gamma,\beta,w}^4 \quad (2r_D r_T r_V^2) \quad (10865)$$

$$\tau_{\gamma,\alpha,w}^6 = \sum_{\delta \in A} Z_{\delta,\gamma}^* \tau_{\delta,\alpha,w}^5 \quad (2r_D r_T^2 r_V) \quad (10866)$$

$$\tau_{\gamma,\alpha}^7 = \sum_{a \in V} W_{a,\alpha}^4 Y_{a,\gamma}^1 \quad (2r_T r_V N_v) \quad (10867)$$

$$\tau_{\gamma,\alpha,i}^8 = \sum_{\delta \in A} Y_{i,\delta}^2 Z_{\delta,\gamma} \tau_{\delta,\alpha}^7 \quad (3r_T^2 r_V N_o) \quad (10868)$$

$$\tau_{\gamma,\alpha}^9 = \sum_{i \in O} W_{i,\alpha}^3 Y_{i,\gamma}^4 \quad (2r_T r_V N_o) \quad (10869)$$

$$\tau_{\gamma,\delta,w,i}^{10} = \sum_{\alpha \in B} \tau_{\gamma,\alpha}^9 \tau_{\delta,\alpha,w}^6 \tau_{\gamma,\alpha,i}^8 \quad (3r_D r_T^2 r_V N_o) \quad (10870)$$

$$\tau_{\gamma,\delta,w}^{11} = \sum_{i \in O} {}^2D_{i,w}^4 Y_{i,\delta}^{4,*} \tau_{\gamma,\delta,w,i}^{10} \quad (3r_D r_T^2 N_o) \quad (10871)$$

$${}^2R_{a,\gamma}^3 \leftarrow \sum_{\delta \in A} \sum_{w \in D} \frac{1}{4} {}^2D_{a,w}^3 Y_{a,\delta}^3 \tau_{\delta,\gamma,w}^{11} \quad (3r_D r_T^2 N_v) \quad (10872)$$

## XI. THC-RCCSD DOUBLES ( $Y^4$ FACTOR) EQUATION

Here expressions for a THC-RCCSD doubles residual, projected against all factors except  $Y^4$ , are given along with their cost

### A. Contributions from $H$

Raw expression

$${}^2R_{j,\zeta}^4 \leftarrow \sum_{\gamma \in A} \sum_{i \in O} \sum_{a \in V} \sum_{b \in V} Y_{a,\gamma}^{1,*} Y_{i,\gamma}^{2,*} Z_{\gamma,\zeta}^* Y_{b,\zeta}^{3,*} {}^2D_{a,i,b,j} V_{a,i,b,j} \quad (10873)$$

Factorized expression

$$\tau_{\gamma,\alpha,w}^0 = \sum_{a \in V} {}^2D_{a,w}^3 W_{a,\alpha}^3 Y_{a,\gamma}^{3,*} \quad (3r_D r_T r_V N_v) \quad (10874)$$

$$\tau_{\gamma,\alpha,w}^1 = \sum_{a \in V} {}^2D_{a,w}^1 W_{a,\alpha}^1 Y_{a,\gamma}^{1,*} \quad (3r_D r_T r_V N_v) \quad (10875)$$

$$\tau^2_{\gamma,\alpha,w} = \sum_{i \in O} {}^2D^2_{i,w} W^2_{i,\alpha} Y^{2,*}_{i,\gamma} \quad (3r_D r_T r_V N_o) \quad (10876)$$

$$\tau^5_{\gamma,\alpha,w} = \sum_{a \in V} {}^2D^3_{a,w} W^3_{a,\alpha} Y^{3,*}_{a,\gamma} \quad (3r_D r_T r_V N_v) \quad (10887)$$

$$\tau^3_{\gamma,\alpha,w} = \sum_{\beta \in B} X_{\beta,\alpha} \tau^1_{\gamma,\beta,w} \tau^2_{\gamma,\beta,w} \quad (3r_D r_T r_V^2) \quad (10877)$$

$$\tau^6_{\gamma,w,i} = \sum_{\alpha \in B} W^4_{i,\alpha} \tau^4_{\gamma,\alpha,w} \tau^5_{\gamma,\alpha,w} \quad (3r_D r_T r_V N_o) \quad (10888)$$

$$\tau^4_{\gamma,\alpha,w} = \sum_{\delta \in A} Z^*_{\delta,\gamma} \tau^3_{\delta,\alpha,w} \quad (2r_D r_T^2 r_V) \quad (10878)$$

$${}^2R^4_{i,\gamma} \leftarrow \sum_{w \in D} {}^2D^4_{i,w} \tau^6_{\gamma,w,i} \quad (2r_D r_T N_o) \quad (10889)$$

Raw expression

$$\tau^5_{\gamma,w,i} = \sum_{\alpha \in B} W^4_{i,\alpha} \tau^0_{\gamma,\alpha,w} \tau^4_{\gamma,\alpha,w} \quad (3r_D r_T r_V N_o) \quad (10879)$$

$${}^2R^4_{j,\zeta} \leftarrow - \sum_{\gamma \in A} \sum_{i \in O} \sum_{k \in O} \sum_{a \in V} \sum_{b \in V} {}^1T_{b,k} Y^{1,*}_{a,\gamma} Y^{2,*}_{i,\gamma} Z^*_{\gamma,\zeta} Y^{3,*}_{b,\zeta} {}^2D^{a,i,b,j}_{a,i,k,j} V_{a,i,k,j} \quad (10890)$$

$${}^2R^4_{i,\gamma} \leftarrow \sum_{w \in D} {}^2D^4_{i,w} \tau^5_{\gamma,w,i} \quad (2r_D r_T N_o) \quad (10880)$$

Factorized expression

$$\tau^0_{\alpha,i} = \sum_{a \in V} {}^1T_{a,i} W^4_{a,\alpha} \quad (2r_V N_o N_v) \quad (10891)$$

## B. Contributions from $(H^1 T)_c$

Raw expression

$${}^2R^4_{j,\zeta} \leftarrow - \sum_{\gamma \in A} \sum_{i \in O} \sum_{k \in O} \sum_{a \in V} \sum_{b \in V} {}^1T_{a,k} Y^{1,*}_{a,\gamma} Y^{2,*}_{i,\gamma} Z^*_{\gamma,\zeta} Y^{3,*}_{b,\zeta} {}^2D^{a,i,b,j}_{b,j,k,i} V_{b,j,k,i} \quad (10881)$$

$$\tau^1_{\gamma,\alpha,w} = \sum_{a \in V} {}^2D^3_{a,w} W^3_{a,\alpha} Y^{3,*}_{a,\gamma} \quad (3r_D r_T r_V N_v) \quad (10892)$$

Factorized expression

$$\tau^2_{\gamma,\alpha,w} = \sum_{a \in V} {}^2D^1_{a,w} W^1_{a,\alpha} Y^{1,*}_{a,\gamma} \quad (3r_D r_T r_V N_v) \quad (10893)$$

$$\tau^0_{\alpha,i} = \sum_{a \in V} {}^1T_{a,i} W^2_{a,\alpha} \quad (2r_V N_o N_v) \quad (10882)$$

$$\tau^3_{\gamma,\alpha,w} = \sum_{i \in O} {}^2D^2_{i,w} W^2_{i,\alpha} Y^{2,*}_{i,\gamma} \quad (3r_D r_T r_V N_o) \quad (10894)$$

$$\tau^1_{\gamma,\alpha,w} = \sum_{i \in O} {}^2D^2_{i,w} Y^{2,*}_{i,\gamma} \tau^0_{\alpha,i} \quad (3r_D r_T r_V N_o) \quad (10883)$$

$$\tau^4_{\gamma,\alpha,w} = \sum_{\beta \in B} X_{\beta,\alpha} \tau^2_{\gamma,\beta,w} \tau^3_{\gamma,\beta,w} \quad (3r_D r_T r_V^2) \quad (10895)$$

$$\tau^2_{\gamma,\alpha,w} = \sum_{a \in V} {}^2D^1_{a,w} W^1_{a,\alpha} Y^{1,*}_{a,\gamma} \quad (3r_D r_T r_V N_v) \quad (10884)$$

$$\tau^5_{\gamma,\alpha,w} = \sum_{\delta \in A} Z^*_{\delta,\gamma} \tau^4_{\delta,\alpha,w} \quad (2r_D r_T^2 r_V) \quad (10896)$$

$$\tau^3_{\gamma,\alpha,w} = \sum_{\beta \in B} X_{\beta,\alpha} \tau^1_{\gamma,\beta,w} \tau^2_{\gamma,\beta,w} \quad (3r_D r_T r_V^2) \quad (10885)$$

$$\tau^6_{\gamma,w,i} = \sum_{\alpha \in B} \tau^0_{\alpha,i} \tau^1_{\gamma,\alpha,w} \tau^5_{\gamma,\alpha,w} \quad (3r_D r_T r_V N_o) \quad (10897)$$

$$\tau^4_{\gamma,\alpha,w} = \sum_{\delta \in A} Z^*_{\delta,\gamma} \tau^3_{\delta,\alpha,w} \quad (2r_D r_T^2 r_V) \quad (10886)$$

$${}^2R^4_{i,\gamma} \leftarrow \sum_{w \in D} {}^2D^4_{i,w} \tau^6_{\gamma,w,i} \quad (2r_D r_T N_o) \quad (10898)$$

Raw expression

$${}^2R^4_{j,\zeta} \leftarrow \sum_{\gamma \in A} \sum_{i \in O} \sum_{a \in V} \sum_{b \in V} \sum_{c \in V} {}^1T_{c,i} Y^{1,*}_{a,\gamma} Y^{2,*}_{i,\gamma} Z^*_{\gamma,\zeta} Y^{3,*}_{b,\zeta} {}^2D^{a,i,b,j} V_{a,c,b,j} \quad (10899)$$

Factorized expression

$$\tau^0_{\gamma,\alpha,w} = \sum_{a \in V} {}^2D^3_{a,w} W^1_{a,\alpha} Y^{3,*}_{a,\gamma} \quad (3r_D r_T r_V N_v) \quad (10900)$$

$$\tau^1_{\gamma,w,i} = \sum_{a \in V} {}^2D^1_{a,w} {}^1T_{a,i} Y^{1,*}_{a,\gamma} \quad (3r_D r_T N_o N_v) \quad (10901)$$

$$\tau^2_{\gamma,\alpha,w} = \sum_{i \in O} W^3_{i,\alpha} \tau^1_{\gamma,w,i} \quad (2r_D r_T r_V N_o) \quad (10902)$$

$$\tau^3_{\gamma,\alpha,w} = \sum_{i \in O} {}^2D^2_{i,w} W^4_{i,\alpha} Y^{2,*}_{i,\gamma} \quad (3r_D r_T r_V N_o) \quad (10903)$$

$$\tau^4_{\gamma,\alpha,w} = \sum_{\beta \in B} X_{\alpha,\beta} \tau^2_{\gamma,\beta,w} \tau^3_{\gamma,\beta,w} \quad (3r_D r_T r_V^2) \quad (10904)$$

$$\tau^5_{\gamma,\alpha,w} = \sum_{\delta \in A} Z^*_{\delta,\gamma} \tau^4_{\delta,\alpha,w} \quad (2r_D r_T^2 r_V) \quad (10905)$$

$$\tau^6_{\gamma,w,i} = \sum_{\alpha \in B} W^2_{i,\alpha} \tau^0_{\gamma,\alpha,w} \tau^5_{\gamma,\alpha,w} \quad (3r_D r_T r_V N_o) \quad (10906)$$

$${}^2R^4_{i,\gamma} \leftarrow - \sum_{w \in D} {}^2D^4_{i,w} \tau^6_{\gamma,w,i} \quad (2r_D r_T N_o) \quad (10907)$$

Raw expression

$${}^2R^4_{j,\zeta} \leftarrow \sum_{\gamma \in A} \sum_{i \in O} \sum_{a \in V} \sum_{b \in V} \sum_{c \in V} {}^1T_{c,j} Y^{1,*}_{a,\gamma} Y^{2,*}_{i,\gamma} Z^*_{\gamma,\zeta} Y^{3,*}_{b,\zeta} {}^2D^{a,i,b,j} V_{a,i,b,c} \quad (10908)$$

Factorized expression

$$\tau^0_{\gamma,\alpha,w} = \sum_{a \in V} {}^2D^1_{a,w} W^1_{a,\alpha} Y^{1,*}_{a,\gamma} \quad (3r_D r_T r_V N_v) \quad (10909)$$

$$\tau^1_{\gamma,\alpha,w} = \sum_{i \in O} {}^2D^2_{i,w} W^2_{i,\alpha} Y^{2,*}_{i,\gamma} \quad (3r_D r_T r_V N_o) \quad (10910)$$

$$\tau^2_{\gamma,\alpha,w} = \sum_{\beta \in B} X_{\beta,\alpha} \tau^0_{\gamma,\beta,w} \tau^1_{\gamma,\beta,w} \quad (3r_D r_T r_V^2) \quad (10911)$$

$$\tau^3_{\gamma,\alpha,w} = \sum_{\delta \in A} Z^*_{\delta,\gamma} \tau^2_{\delta,\alpha,w} \quad (2r_D r_T^2 r_V) \quad (10912)$$

$$\tau^4_{\gamma,w,i} = \sum_{a \in V} {}^2D^3_{a,w} {}^1T_{a,i} Y^{3,*}_{a,\gamma} \quad (3r_D r_T N_o N_v) \quad (10913)$$

$$\tau^5_{\gamma,\alpha,w} = \sum_{i \in O} W^3_{i,\alpha} \tau^4_{\gamma,w,i} \quad (2r_D r_T r_V N_o) \quad (10914)$$

$$\tau^6_{\gamma,w,i} = \sum_{\alpha \in B} W^4_{i,\alpha} \tau^3_{\gamma,\alpha,w} \tau^5_{\gamma,\alpha,w} \quad (3r_D r_T r_V N_o) \quad (10915)$$

$${}^2R^4_{i,\gamma} \leftarrow - \sum_{w \in D} {}^2D^4_{i,w} \tau^6_{\gamma,w,i} \quad (2r_D r_T N_o) \quad (10916)$$

### C. Contributions from $(H^1 T^1 T)_c$

Raw expression

$${}^2R^4_{j,\zeta} \leftarrow \sum_{\gamma \in A} \sum_{i \in O} \sum_{a \in V} \sum_{b \in V} \sum_{c \in V} \sum_{d \in V} {}^1T_{c,i} {}^1T_{d,j} Y^{1,*}_{a,\gamma} Y^{2,*}_{i,\gamma} Z^*_{\gamma,\zeta} Y^{3,*}_{b,\zeta} {}^2D^{a,i,b,j} V_{a,c,b,d} \quad (10917)$$

Factorized expression

$$\tau^0_{\gamma,\alpha,w} = \sum_{a \in V} {}^2D^3_{a,w} W^1_{a,\alpha} Y^{3,*}_{a,\gamma} \quad (3r_D r_T r_V N_v) \quad (10918)$$

$$\tau^1_{\alpha,i} = \sum_{a \in V} {}^1T_{a,i} W^4_{a,\alpha} \quad (2r_V N_o N_v) \quad (10919)$$

$$\tau^2_{\gamma,\alpha,w} = \sum_{i \in O} {}^2D^2_{i,w} Y^{2,*}_{i,\gamma} \tau^1_{\alpha,i} \quad (3r_D r_T r_V N_o) \quad (10920)$$

$$\tau^3_{\gamma,w,i} = \sum_{a \in V} {}^2D^1_{a,w} {}^1T_{a,i} Y^{1,*}_{a,\gamma} \quad (3r_D r_T N_o N_v) \quad (10921)$$

$$\tau^4_{\gamma,\alpha,w} = \sum_{i \in O} W^3_{i,\alpha} \tau^3_{\gamma,w,i} \quad (2r_D r_T r_V N_o) \quad (10922)$$

$$\tau^5_{\gamma,\alpha,w} = \sum_{\beta \in B} X_{\alpha,\beta} \tau^2_{\gamma,\beta,w} \tau^4_{\gamma,\beta,w} \quad (3r_D r_T r_V^2) \quad (10923)$$

$$\tau^6_{\gamma,\alpha,w} = \sum_{\delta \in A} Z^*_{\delta,\gamma} \tau^5_{\delta,\alpha,w} \quad (2r_D r_T^2 r_V) \quad (10924)$$

$$\tau^7_{\gamma,w,i} = \sum_{\alpha \in B} W^2_{i,\alpha} \tau^0_{\gamma,\alpha,w} \tau^6_{\gamma,\alpha,w} \quad (3r_D r_T r_V N_o) \quad (10925)$$

$${}^2R^4_{i,\gamma} \leftarrow - \sum_{w \in D} {}^2D^4_{i,w} \tau^7_{\gamma,w,i} \quad (2r_D r_T N_o) \quad (10926)$$

Raw expression

$${}^2R^4_{j,\zeta} \leftarrow \sum_{\gamma \in A} \sum_{i \in O} \sum_{k \in O} \sum_{l \in O} \sum_{a \in V} \sum_{b \in V} {}^1T_{a,k} {}^1T_{b,l} Y^{1,*}_{a,\gamma} Y^{2,*}_{i,\gamma} Z^*_{\gamma,\zeta} Y^{3,*}_{b,\zeta} {}^2D^{a,i,b,j} V_{k,i,l,j} \quad (10927)$$

Factorized expression

$$\tau^0_{\gamma,\alpha,w} = \sum_{a \in V} {}^2D^3_{a,w} W^1_{a,\alpha} Y^{3,*}_{a,\gamma} \quad (3r_D r_T r_V N_v) \quad (10928)$$

$$\tau^1_{\gamma,w,i} = \sum_{a \in V} {}^2D^1_{a,w} {}^1T_{a,i} Y^{1,*}_{a,\gamma} \quad (3r_D r_T N_o N_v) \quad (10929)$$

$$\tau^2_{\gamma,\alpha,w} = \sum_{i \in O} W^3_{i,\alpha} \tau^1_{\gamma,w,i} \quad (2r_D r_T r_V N_o) \quad (10930)$$

$$\tau^3_{\gamma,\alpha,w} = \sum_{i \in O} {}^2D^2_{i,w} W^4_{i,\alpha} Y^{2,*}_{i,\gamma} \quad (3r_D r_T r_V N_o) \quad (10931)$$

$$\tau^4_{\gamma,\alpha,w} = \sum_{\beta \in B} X_{\alpha,\beta} \tau^2_{\gamma,\beta,w} \tau^3_{\gamma,\beta,w} \quad (3r_D r_T r_V^2) \quad (10932)$$

$$\tau^5_{\gamma,\alpha,w} = \sum_{\delta \in A} Z^*_{\delta,\gamma} \tau^4_{\delta,\alpha,w} \quad (2r_D r_T^2 r_V) \quad (10933)$$

$$\tau^6_{\alpha,i} = \sum_{a \in V} {}^1T_{a,i} W^2_{a,\alpha} \quad (2r_V N_o N_v) \quad (10934)$$

$$\tau^7_{\gamma,w,i} = \sum_{\alpha \in B} \tau^6_{\alpha,i} \tau^0_{\gamma,\alpha,w} \tau^5_{\gamma,\alpha,w} \quad (3r_D r_T r_V N_o) \quad (10935)$$

$${}^2R^4_{i,\gamma} \leftarrow - \sum_{w \in D} {}^2D^4_{i,w} \tau^7_{\gamma,w,i} \quad (2r_D r_T N_o) \quad (10936)$$

Raw expression

$${}^2R^4_{j,\zeta} \leftarrow - \sum_{\gamma \in A} \sum_{i \in O} \sum_{k \in O} \sum_{a \in V} \sum_{b \in V} \sum_{c \in V} {}^1T_{a,k} {}^1T_{c,i} Y^{1,*}_{a,\gamma} Y^{2,*}_{i,\gamma} Z^*_{\gamma,\zeta} Y^{3,*}_{b,\zeta} {}^2D^{a,i,b,j} V_{b,j,k,c} \quad (10937)$$

Factorized expression

$$\tau^0_{\gamma,w,i} = \sum_{a \in V} {}^2D^3_{a,w} {}^1T_{a,i} Y^{3,*}_{a,\gamma} \quad (3r_D r_T N_o N_v) \quad (10938)$$

$$\tau^1_{\gamma,\alpha,w} = \sum_{i \in O} W^3_{i,\alpha} \tau^0_{\gamma,w,i} \quad (2r_D r_T r_V N_o) \quad (10939)$$

$$\tau^2_{\alpha,i} = \sum_{a \in V} {}^1T_{a,i} W^2_{a,\alpha} \quad (2r_V N_o N_v) \quad (10940)$$

$$\tau^3_{\gamma,\alpha,w} = \sum_{i \in O} {}^2D^2_{i,w} Y^{2,*}_{i,\gamma} \tau^2_{\alpha,i} \quad (3r_D r_T r_V N_o) \quad (10941)$$

$$\tau^4_{\gamma,\alpha,w} = \sum_{a \in V} {}^2D^1_{a,w} W^1_{a,\alpha} Y^{1,*}_{a,\gamma} \quad (3r_D r_T r_V N_v) \quad (10942)$$

$$\tau^5_{\gamma,\alpha,w} = \sum_{\beta \in B} X_{\beta,\alpha} \tau^3_{\gamma,\beta,w} \tau^4_{\gamma,\beta,w} \quad (3r_D r_T r_V^2) \quad (10943)$$

$$\tau^6_{\gamma,\alpha,w} = \sum_{\delta \in A} Z^*_{\delta,\gamma} \tau^5_{\delta,\alpha,w} \quad (2r_D r_T^2 r_V) \quad (10944)$$

$$\tau_{\gamma,w,i}^7 = \sum_{\alpha \in B} W_{i,\alpha}^4 \tau_{\gamma,\alpha,w}^1 \tau_{\gamma,\alpha,w}^6 \quad (3r_D r_T r_V N_o) \quad (10945)$$

$${}^2R_{i,\gamma}^4 \leftarrow - \sum_{w \in D} {}^2D_{i,w}^4 \tau_{\gamma,w,i}^7 \quad (2r_D r_T N_o) \quad (10946)$$

Raw expression

$${}^2R_{j,\zeta}^4 \leftarrow - \sum_{\gamma \in A} \sum_{i \in O} \sum_{k \in O} \sum_{a \in V} \sum_{b \in V} \sum_{c \in V} {}^1T_{a,k} {}^1T_{c,j} Y_{a,\gamma}^{1,*} Y_{i,\gamma}^{2,*} Z_{\gamma,\zeta}^* Y_{b,\zeta}^{3,*} {}^2D_{a,i,b,j} V_{b,c,k,i} \quad (10947)$$

Factorized expression

$$\tau_{\gamma,\alpha,w}^0 = \sum_{a \in V} {}^2D_{a,w}^1 W_{a,\alpha}^1 Y_{a,\gamma}^{1,*} \quad (3r_D r_T r_V N_v) \quad (10948)$$

$$\tau_{\gamma,\alpha,w}^1 = \sum_{i \in O} {}^2D_{i,w}^2 W_{i,\alpha}^2 Y_{i,\gamma}^{2,*} \quad (3r_D r_T r_V N_o) \quad (10949)$$

$$\tau_{\gamma,\alpha,w}^2 = \sum_{\beta \in B} X_{\beta,\alpha} \tau_{\gamma,\beta,w}^0 \tau_{\gamma,\beta,w}^1 \quad (3r_D r_T r_V^2) \quad (10950)$$

$$\tau_{\gamma,\alpha,w}^3 = \sum_{\delta \in A} Z_{\delta,\gamma}^* \tau_{\delta,\alpha,w}^2 \quad (2r_D r_T^2 r_V) \quad (10951)$$

$$\tau_{\gamma,w,i}^4 = \sum_{a \in V} {}^2D_{a,w}^3 {}^1T_{a,i} Y_{a,\gamma}^{3,*} \quad (3r_D r_T N_o N_v) \quad (10952)$$

$$\tau_{\gamma,\alpha,w}^5 = \sum_{i \in O} W_{i,\alpha}^3 \tau_{\gamma,w,i}^4 \quad (2r_D r_T r_V N_o) \quad (10953)$$

$$\tau_{\alpha,i}^6 = \sum_{a \in V} {}^1T_{a,i} W_{a,\alpha}^4 \quad (2r_V N_o N_v) \quad (10954)$$

$$\tau_{\gamma,w,i}^7 = \sum_{\alpha \in B} \tau_{\alpha,i}^6 \tau_{\gamma,\alpha,w}^3 \tau_{\gamma,\alpha,w}^5 \quad (3r_D r_T r_V N_o) \quad (10955)$$

$${}^2R_{i,\gamma}^4 \leftarrow - \sum_{w \in D} {}^2D_{i,w}^4 \tau_{\gamma,w,i}^7 \quad (2r_D r_T N_o) \quad (10956)$$

Raw expression

$${}^2R_{j,\zeta}^4 \leftarrow - \sum_{\gamma \in A} \sum_{i \in O} \sum_{k \in O} \sum_{a \in V} \sum_{b \in V} \sum_{c \in V} {}^1T_{b,k} {}^1T_{c,i} Y_{a,\gamma}^{1,*} Y_{i,\gamma}^{2,*} Z_{\gamma,\zeta}^* Y_{b,\zeta}^{3,*} {}^2D_{a,i,b,j} V_{a,c,k,j} \quad (10957)$$

Factorized expression

$$\tau_{\alpha,i}^0 = \sum_{a \in V} {}^1T_{a,i} W_{a,\alpha}^2 \quad (2r_V N_o N_v) \quad (10958)$$

$$\tau_{\gamma,\alpha,w}^1 = \sum_{i \in O} {}^2D_{i,w}^2 Y_{i,\gamma}^{2,*} \tau_{\alpha,i}^0 \quad (3r_D r_T r_V N_o) \quad (10959)$$

$$\tau_{\gamma,\alpha,w}^2 = \sum_{a \in V} {}^2D_{a,w}^1 W_{a,\alpha}^1 Y_{a,\gamma}^{1,*} \quad (3r_D r_T r_V N_v) \quad (10960)$$

$$\tau_{\gamma,\alpha,w}^3 = \sum_{\beta \in B} X_{\beta,\alpha} \tau_{\gamma,\beta,w}^1 \tau_{\gamma,\beta,w}^2 \quad (3r_D r_T r_V^2) \quad (10961)$$

$$\tau_{\gamma,\alpha,w}^4 = \sum_{\delta \in A} Z_{\delta,\gamma}^* \tau_{\delta,\alpha,w}^3 \quad (2r_D r_T^2 r_V) \quad (10962)$$

$$\tau_{\gamma,\alpha,w}^5 = \sum_{a \in V} {}^2D_{a,w}^3 W_{a,\alpha}^3 Y_{a,\gamma}^{3,*} \quad (3r_D r_T r_V N_v) \quad (10963)$$

$$\tau_{\alpha,i}^6 = \sum_{a \in V} {}^1T_{a,i} W_{a,\alpha}^4 \quad (2r_V N_o N_v) \quad (10964)$$

$$\tau_{\gamma,w,i}^7 = \sum_{\alpha \in B} \tau_{\alpha,i}^6 \tau_{\gamma,\alpha,w}^4 \tau_{\gamma,\alpha,w}^5 \quad (3r_D r_T r_V N_o) \quad (10965)$$

$${}^2R_{i,\gamma}^4 \leftarrow - \sum_{w \in D} {}^2D_{i,w}^4 \tau_{\gamma,w,i}^7 \quad (2r_D r_T N_o) \quad (10966)$$

Raw expression

$${}^2R_{j,\zeta}^4 \leftarrow - \sum_{\gamma \in A} \sum_{i \in O} \sum_{k \in O} \sum_{a \in V} \sum_{b \in V} \sum_{c \in V} {}^1T_{b,k} {}^1T_{c,j} Y_{a,\gamma}^{1,*} Y_{i,\gamma}^{2,*} Z_{\gamma,\zeta}^* Y_{b,\zeta}^{3,*} {}^2D_{a,i,b,j} V_{a,i,k,c} \quad (10967)$$

Factorized expression

$$\tau^0_{\gamma,w,i} = \sum_{a \in V} {}^2D^3_{a,w} {}^1T_{a,i} Y^{3,*}_{a,\gamma} \quad (3r_D r_T N_o N_v) \quad (10968)$$

$$\tau^1_{\gamma,\alpha,w} = \sum_{a \in V} {}^2D^1_{a,w} W^1_{a,\alpha} Y^{1,*}_{a,\gamma} \quad (3r_D r_T r_V N_v) \quad (10979)$$

$$\tau^1_{\gamma,\alpha,w} = \sum_{i \in O} W^3_{i,\alpha} \tau^0_{\gamma,w,i} \quad (2r_D r_T r_V N_o) \quad (10969)$$

$$\tau^2_{\gamma,\alpha,w} = \sum_{i \in O} {}^2D^2_{i,w} W^2_{i,\alpha} Y^{2,*}_{i,\gamma} \quad (3r_D r_T r_V N_o) \quad (10980)$$

$$\tau^2_{\gamma,w,i} = \sum_{a \in V} {}^2D^1_{a,w} {}^1T_{a,i} Y^{1,*}_{a,\gamma} \quad (3r_D r_T N_o N_v) \quad (10970)$$

$$\tau^3_{\gamma,\alpha} = \sum_{a \in V} W^4_{a,\alpha} Y^3_{a,\gamma} \quad (2r_T r_V N_v) \quad (10981)$$

$$\tau^3_{\gamma,\alpha,w} = \sum_{i \in O} W^1_{i,\alpha} \tau^2_{\gamma,w,i} \quad (2r_D r_T r_V N_o) \quad (10971)$$

$$\tau^4_{\gamma,\alpha} = \sum_{i \in O} W^3_{i,\alpha} Y^4_{i,\gamma} \quad (2r_T r_V N_o) \quad (10982)$$

$$\tau^4_{\gamma,\alpha,w} = \sum_{i \in O} {}^2D^2_{i,w} W^2_{i,\alpha} Y^{2,*}_{i,\gamma} \quad (3r_D r_T r_V N_o) \quad (10972)$$

$$\tau^5_{\gamma,\alpha} = \sum_{\beta \in B} X_{\alpha,\beta} \tau^3_{\gamma,\beta} \tau^4_{\gamma,\beta} \quad (3r_T r_V^2) \quad (10983)$$

$$\tau^5_{\gamma,\alpha,w} = \sum_{\beta \in B} X_{\beta,\alpha} \tau^3_{\gamma,\beta,w} \tau^4_{\gamma,\beta,w} \quad (3r_D r_T r_V^2) \quad (10973)$$

$$\tau^6_{\gamma,\alpha} = \sum_{\delta \in A} Z_{\gamma,\delta} \tau^5_{\delta,\alpha} \quad (2r_T^2 r_V) \quad (10984)$$

$$\tau^6_{\gamma,\alpha,w} = \sum_{\delta \in A} Z^*_{\delta,\gamma} \tau^5_{\delta,\alpha,w} \quad (2r_D r_T^2 r_V) \quad (10974)$$

$$\tau^7_{\gamma,\delta,w} = \sum_{\alpha \in B} \tau^6_{\gamma,\alpha} \tau^1_{\delta,\alpha,w} \tau^2_{\delta,\alpha,w} \quad (3r_D r_T^2 r_V) \quad (10985)$$

$$\tau^7_{\gamma,w,i} = \sum_{\alpha \in B} W^4_{i,\alpha} \tau^1_{\gamma,\alpha,w} \tau^6_{\gamma,\alpha,w} \quad (3r_D r_T r_V N_o) \quad (10975)$$

$$\tau^8_{\gamma,\delta,w} = \sum_{\epsilon \in A} Z^*_{\epsilon,\delta} \tau^7_{\gamma,\epsilon,w} \quad (2r_D r_T^3) \quad (10986)$$

$${}^2R^4_{i,\gamma} \leftarrow \sum_{w \in D} {}^2D^4_{i,w} \tau^7_{\gamma,w,i} \quad (2r_D r_T N_o) \quad (10976)$$

$${}^2R^4_{i,\gamma} \leftarrow \sum_{\delta \in A} \sum_{w \in D} {}^2D^4_{i,w} Y^2_{i,\delta} \tau^0_{\delta,\gamma,w} \tau^8_{\delta,\gamma,w} \quad (4r_D r_T^2 N_o) \quad (10987)$$

#### D. Contributions from $(H^2 T)_c$

Raw expression

$${}^2R^4_{j,\zeta} \leftarrow \sum_{\gamma \in A} \sum_{i \in O} \sum_{a \in V} \sum_{b \in V} \sum_{c \in V} \sum_{d \in V} \frac{1}{2} Y^{1,*}_{a,\gamma} Y^{2,*}_{i,\gamma} Z^*_{\gamma,\zeta} Y^{3,*}_{b,\zeta} {}^2D^{a,i,b,j} {}^2T_{c,i,d,j} V_{a,c,b,d} \quad (10977)$$

Factorized expression

$$\tau^0_{\gamma,\delta,w} = \sum_{a \in V} {}^2D^3_{a,w} Y^1_{a,\gamma} Y^{3,*}_{a,\delta} \quad (3r_D r_T^2 N_v) \quad (10978)$$

Raw expression

$${}^2R^4_{j,\zeta} \leftarrow \sum_{\gamma \in A} \sum_{i \in O} \sum_{a \in V} \sum_{b \in V} \sum_{c \in V} \sum_{d \in V} \frac{1}{2} Y^{1,*}_{a,\gamma} Y^{2,*}_{i,\gamma} Z^*_{\gamma,\zeta} Y^{3,*}_{b,\zeta} {}^2D^{a,i,b,j} {}^2T_{c,j,d,i} V_{a,d,b,c} \quad (10988)$$

Factorized expression

$$\tau^0_{\gamma,\delta,w} = \sum_{a \in V} {}^2D^3_{a,w} Y^3_{a,\gamma} Y^{3,*}_{a,\delta} \quad (3r_D r_T^2 N_v) \quad (10989)$$

$$\tau^1_{\gamma,\alpha,w} = \sum_{a \in V} {}^2D^1_{a,w} W^1_{a,\alpha} Y^{1,*}_{a,\gamma} \quad (3r_D r_T r_V N_v) \quad (10990)$$



$$\tau^2_{\gamma,\alpha,w} = \sum_{i \in O} {}^2D^2_{i,w} W^2_{i,\alpha} Y^{2,*}_{i,\gamma} \quad (3r_D r_T r_V N_o) \quad (10991)$$

$$\tau^3_{\gamma,\alpha} = \sum_{a \in V} W^4_{a,\alpha} Y^1_{a,\gamma} \quad (2r_T r_V N_v) \quad (10992)$$

$$\tau^4_{\gamma,\alpha} = \sum_{i \in O} W^3_{i,\alpha} Y^2_{i,\gamma} \quad (2r_T r_V N_o) \quad (10993)$$

$$\tau^5_{\gamma,\alpha} = \sum_{\beta \in B} X_{\alpha,\beta} \tau^3_{\gamma,\beta} \tau^4_{\gamma,\beta} \quad (3r_T r_V^2) \quad (10994)$$

$$\tau^6_{\gamma,\alpha} = \sum_{\delta \in A} Z_{\delta,\gamma} \tau^5_{\delta,\alpha} \quad (2r_T^2 r_V) \quad (10995)$$

$$\tau^7_{\gamma,\delta,w} = \sum_{\alpha \in B} \tau^6_{\gamma,\alpha} \tau^1_{\delta,\alpha,w} \tau^2_{\delta,\alpha,w} \quad (3r_D r_T^2 r_V) \quad (10996)$$

$$\tau^8_{\gamma,\delta,w} = \sum_{\epsilon \in A} Z^*_{\epsilon,\delta} \tau^7_{\gamma,\epsilon,w} \quad (2r_D r_T^3) \quad (10997)$$

$${}^2R^4_{i,\gamma} \leftarrow \sum_{\delta \in A} \sum_{w \in D} {}^2D^4_{i,w} Y^4_{i,\delta} \tau^0_{\delta,\gamma,w} \tau^8_{\delta,\gamma,w} \quad (4r_D r_T^2 N_o) \quad (10998)$$

Raw expression

$${}^2R^4_{j,\zeta} \leftarrow - \sum_{\gamma \in A} \sum_{i \in O} \sum_{k \in O} \sum_{a \in V} \sum_{b \in V} \frac{1}{2} Y^{1,*}_{a,\gamma} Y^{2,*}_{i,\gamma} Z^*_{\gamma,\zeta} Y^{3,*}_{b,\zeta} f_{k,i} {}^2D^{a,i,b,j} {}^2T_{a,k,b,j} \quad (10999)$$

Factorized expression

$$\tau^0_{\gamma,\alpha,w} = \sum_{a \in V} {}^2D^3_{a,w} W^1_{a,\alpha} Y^{3,*}_{a,\gamma} \quad (3r_D r_T r_V N_v) \quad (11000)$$

$$\tau^1_{\gamma,\alpha} = \sum_{a \in V} W^4_{a,\alpha} Y^3_{a,\gamma} \quad (2r_T r_V N_v) \quad (11001)$$

$$\tau^2_{\gamma,\alpha} = \sum_{i \in O} W^3_{i,\alpha} Y^4_{i,\gamma} \quad (2r_T r_V N_o) \quad (11002)$$

$$\tau^3_{\gamma,\alpha} = \sum_{\beta \in B} X_{\alpha,\beta} \tau^1_{\gamma,\beta} \tau^2_{\gamma,\beta} \quad (3r_T r_V^2) \quad (11003)$$

$$\tau^4_{\gamma,\alpha} = \sum_{\delta \in A} Z_{\gamma,\delta} \tau^3_{\delta,\alpha} \quad (2r_T^2 r_V) \quad (11004)$$

$$\tau^5_{\gamma,\delta,w} = \sum_{a \in V} {}^2D^1_{a,w} Y^1_{a,\gamma} Y^{1,*}_{a,\delta} \quad (3r_D r_T^2 N_v) \quad (11005)$$

$$\tau^6_{\gamma,\delta,w} = \sum_{i \in O} {}^2D^2_{i,w} Y^2_{i,\gamma} Y^{2,*}_{i,\delta} \quad (3r_D r_T^2 N_o) \quad (11006)$$

$$\tau^7_{\gamma,\delta,w} = \sum_{\epsilon \in A} Z^*_{\epsilon,\delta} \tau^5_{\gamma,\epsilon,w} \tau^6_{\gamma,\epsilon,w} \quad (3r_D r_T^3) \quad (11007)$$

$$\tau^8_{\gamma,\alpha,w} = \sum_{\delta \in A} \tau^4_{\delta,\alpha} \tau^7_{\delta,\gamma,w} \quad (2r_D r_T^2 r_V) \quad (11008)$$

$$\tau^9_{\gamma,w,i} = \sum_{\alpha \in B} W^2_{i,\alpha} \tau^0_{\gamma,\alpha,w} \tau^8_{\gamma,\alpha,w} \quad (3r_D r_T r_V N_o) \quad (11009)$$

$${}^2R^4_{i,\gamma} \leftarrow \sum_{w \in D} {}^2D^4_{i,w} \tau^9_{\gamma,w,i} \quad (2r_D r_T N_o) \quad (11010)$$

Raw expression

$${}^2R^4_{j,\zeta} \leftarrow - \sum_{\gamma \in A} \sum_{i \in O} \sum_{k \in O} \sum_{a \in V} \sum_{b \in V} \frac{1}{2} Y^{1,*}_{a,\gamma} Y^{2,*}_{i,\gamma} Z^*_{\gamma,\zeta} Y^{3,*}_{b,\zeta} f_{k,i} {}^2D^{a,i,b,j} {}^2T_{b,j,a,k} \quad (11011)$$

Factorized expression

$$\tau^0_{\gamma,\alpha,w} = \sum_{a \in V} {}^2D^3_{a,w} W^1_{a,\alpha} Y^{3,*}_{a,\gamma} \quad (3r_D r_T r_V N_v) \quad (11012)$$

$$\tau^1_{\gamma,\delta,w} = \sum_{a \in V} {}^2D^1_{a,w} Y^3_{a,\gamma} Y^{1,*}_{a,\delta} \quad (3r_D r_T^2 N_v) \quad (11013)$$

$$\tau^2_{\gamma,\delta,w} = \sum_{i \in O} {}^2D^2_{i,w} Y^4_{i,\gamma} Y^{2,*}_{i,\delta} \quad (3r_D r_T^2 N_o) \quad (11014)$$

$$\tau^3_{\gamma,\delta,w} = \sum_{\epsilon \in A} Z^*_{\epsilon,\delta} \tau^1_{\gamma,\epsilon,w} \tau^2_{\gamma,\epsilon,w} \quad (3r_D r_T^3) \quad (11015)$$

$$\tau^4_{\gamma,\alpha} = \sum_{a \in V} W^4_{a,\alpha} Y^1_{a,\gamma} \quad (2r_T r_V N_v) \quad (11016)$$

$$\tau^5_{\gamma,\alpha} = \sum_{i \in O} W^3_{i,\alpha} Y^2_{i,\gamma} \quad (2r_T r_V N_o) \quad (11017)$$

$$\tau^6_{\gamma,\alpha} = \sum_{\beta \in B} X_{\alpha,\beta} \tau^4_{\gamma,\beta} \tau^5_{\gamma,\beta} \quad (3r_T r_V^2) \quad (11018)$$

$$\tau^7_{\gamma,\alpha} = \sum_{\delta \in A} Z_{\delta,\gamma} \tau^6_{\delta,\alpha} \quad (2r_T^2 r_V) \quad (11019)$$

$$\tau^8_{\gamma,\alpha,w} = \sum_{\delta \in A} \tau^7_{\delta,\alpha} \tau^3_{\delta,\gamma,w} \quad (2r_D r_T^2 r_V) \quad (11020)$$

$$\tau^9_{\gamma,w,i} = \sum_{\alpha \in B} W^2_{i,\alpha} \tau^0_{\gamma,\alpha,w} \tau^8_{\gamma,\alpha,w} \quad (3r_D r_T r_V N_o) \quad (11021)$$

$${}^2R^4_{i,\gamma} \leftarrow \sum_{w \in D} {}^2D^4_{i,w} \tau^9_{\gamma,w,i} \quad (2r_D r_T N_o) \quad (11022)$$

Raw expression

$${}^2R^4_{j,\zeta} \leftarrow - \sum_{\gamma \in A} \sum_{i \in O} \sum_{k \in O} \sum_{a \in V} \sum_{b \in V} \frac{1}{2} Y^{1,*}_{a,\gamma} Y^{2,*}_{i,\gamma} Z^*_{\gamma,\zeta} Y^{3,*}_{b,\zeta} f_{k,j} {}^2D^{a,i,b,j} {}^2T_{a,i,b,k} \quad (11023)$$

Factorized expression

$$\tau^0_{\gamma,\delta,w} = \sum_{a \in V} {}^2D^3_{a,w} Y^1_{a,\gamma} Y^{3,*}_{a,\delta} \quad (3r_D r_T^2 N_v) \quad (11024)$$

$$\tau^1_{\alpha,i,j} = \sum_{\beta \in B} X_{\alpha,\beta} W^3_{i,\beta} W^4_{j,\beta} \quad (3r_V^2 N_o^2) \quad (11025)$$

$$\tau^2_{\gamma,\alpha,i} = \sum_{j \in O} Y^4_{j,\gamma} \tau^1_{\alpha,j,i} \quad (2r_T r_V N_o^2) \quad (11026)$$

$$\tau^3_{\gamma,\alpha} = \sum_{a \in V} W^2_{a,\alpha} Y^3_{a,\gamma} \quad (2r_T r_V N_v) \quad (11027)$$

$$\tau^4_{\gamma,i,a} = \sum_{\alpha \in B} W^1_{a,\alpha} \tau^3_{\gamma,\alpha} \tau^2_{\gamma,\alpha,i} \quad (3r_T r_V N_o N_v) \quad (11028)$$

$$\tau^5_{\gamma,\delta,w} = \sum_{i \in O} \sum_{a \in V} {}^2D^1_{a,w} {}^2D^2_{i,w} Y^{1,*}_{a,\delta} Y^{2,*}_{i,\delta} \tau^4_{\gamma,i,a} \quad (5r_D r_T^2 N_o N_v) \quad (11029)$$

$$\tau^6_{\gamma,\delta,w} = \sum_{\epsilon \in A} Z^*_{\epsilon,\delta} \tau^5_{\gamma,\epsilon,w} \quad (2r_D r_T^3) \quad (11030)$$

$$\tau^7_{\gamma,\delta,w} = \sum_{\epsilon \in A} Z_{\gamma,\epsilon} \tau^6_{\epsilon,\delta,w} \quad (2r_D r_T^3) \quad (11031)$$

$${}^2R^4_{i,\gamma} \leftarrow - \sum_{\delta \in A} \sum_{w \in D} \frac{1}{2} {}^2D^4_{i,w} Y^2_{i,\delta} \tau^0_{\delta,\gamma,w} \tau^7_{\delta,\gamma,w} \quad (4r_D r_T^2 N_o) \quad (11032)$$

Raw expression

$${}^2R^4_{j,\zeta} \leftarrow - \sum_{\gamma \in A} \sum_{i \in O} \sum_{k \in O} \sum_{a \in V} \sum_{b \in V} \frac{1}{2} Y^{1,*}_{a,\gamma} Y^{2,*}_{i,\gamma} Z^*_{\gamma,\zeta} Y^{3,*}_{b,\zeta} f_{k,j} {}^2D^{a,i,b,j} {}^2T_{b,k,a,i} \quad (11033)$$

Factorized expression

$$\tau^0_{\gamma,\delta,w} = \sum_{a \in V} {}^2D^3_{a,w} Y^3_{a,\gamma} Y^{3,*}_{a,\delta} \quad (3r_D r_T^2 N_v) \quad (11034)$$

$$\tau^1_{\alpha,i,j} = \sum_{\beta \in B} X_{\alpha,\beta} W^3_{i,\beta} W^4_{j,\beta} \quad (3r_V^2 N_o^2) \quad (11035)$$

$$\tau^2_{\gamma,\alpha,i} = \sum_{j \in O} Y^2_{j,\gamma} \tau^1_{\alpha,j,i} \quad (2r_T r_V N_o^2) \quad (11036)$$

$$\tau^3_{\gamma,\alpha} = \sum_{a \in V} W^2_{a,\alpha} Y^1_{a,\gamma} \quad (2r_T r_V N_v) \quad (11037)$$

$$\tau^4_{\gamma,i,a} = \sum_{\alpha \in B} W^1_{a,\alpha} \tau^3_{\gamma,\alpha} \tau^2_{\gamma,\alpha,i} \quad (3r_T r_V N_o N_v) \quad (11038)$$

$$\tau^5_{\gamma,\delta,w} = \sum_{i \in O} \sum_{a \in V} {}^2D^1_{a,w} {}^2D^2_{i,w} Y^{1,*}_{a,\delta} Y^{2,*}_{i,\delta} \tau^4_{\gamma,i,a} \quad (5r_D r_T^2 N_o N_v) \quad (11039)$$

$$\tau^6_{\gamma,\delta,w} = \sum_{\epsilon \in A} Z^*_{\epsilon,\delta} \tau^5_{\gamma,\epsilon,w} \quad (2r_D r_T^3) \quad (11040)$$

$$\tau^8_{\gamma,\delta,i} = \sum_{\epsilon \in A} \sum_{w \in D} {}^2D^4_{i,w} \tau^0_{\epsilon,\delta,w} \tau^7_{\epsilon,\gamma,w,i} \quad (3r_D r_T^3 N_o) \quad (11052)$$

$$\tau^7_{\gamma,\delta,w} = \sum_{\epsilon \in A} Z_{\epsilon,\gamma} \tau^6_{\epsilon,\delta,w} \quad (2r_D r_T^3) \quad (11041)$$

$${}^2R^4_{i,\gamma} \leftarrow - \sum_{\delta \in A} \frac{1}{2} Z^*_{\delta,\gamma} \tau^8_{\delta,\gamma,i} \quad (2r_T^2 N_o) \quad (11053)$$

$${}^2R^4_{i,\gamma} \leftarrow - \sum_{\delta \in A} \sum_{w \in D} \frac{1}{2} {}^2D^4_{i,w} Y^4_{i,\delta} \tau^0_{\delta,\gamma,w} \tau^7_{\delta,\gamma,w} \quad (4r_D r_T^2 N_o) \quad (11042)$$

Raw expression

$${}^2R^4_{j,\zeta} \leftarrow \sum_{\gamma \in A} \sum_{i \in O} \sum_{k \in O} \sum_{l \in O} \sum_{a \in V} \sum_{b \in V} \frac{1}{2} Y^{1,*}_{a,\gamma} Y^{2,*}_{i,\gamma} Z^*_{\gamma,\zeta} Y^{3,*}_{b,\zeta} {}^2D^{a,i,b,j} {}^2T_{b,k,a,l} V_{l,i,k,j} \quad (11054)$$

Raw expression

$${}^2R^4_{j,\zeta} \leftarrow \sum_{\gamma \in A} \sum_{i \in O} \sum_{k \in O} \sum_{l \in O} \sum_{a \in V} \sum_{b \in V} \frac{1}{2} Y^{1,*}_{a,\gamma} Y^{2,*}_{i,\gamma} Z^*_{\gamma,\zeta} Y^{3,*}_{b,\zeta} {}^2D^{a,i,b,j} {}^2T_{a,k,b,l} V_{k,i,l,j} \quad (11043)$$

Factorized expression

$$\tau^0_{\gamma,\delta,w} = \sum_{a \in V} {}^2D^3_{a,w} Y^3_{a,\gamma} Y^{3,*}_{a,\delta} \quad (3r_D r_T^2 N_v) \quad (11055)$$

Factorized expression

$$\tau^0_{\gamma,\delta,w} = \sum_{a \in V} {}^2D^3_{a,w} Y^1_{a,\gamma} Y^{3,*}_{a,\delta} \quad (3r_D r_T^2 N_v) \quad (11044)$$

$$\tau^1_{\gamma,\alpha,w} = \sum_{a \in V} {}^2D^1_{a,w} W^1_{a,\alpha} Y^{1,*}_{a,\gamma} \quad (3r_D r_T r_V N_v) \quad (11056)$$

$$\tau^1_{\gamma,\alpha,w} = \sum_{a \in V} {}^2D^1_{a,w} W^1_{a,\alpha} Y^{1,*}_{a,\gamma} \quad (3r_D r_T r_V N_v) \quad (11045)$$

$$\tau^2_{\gamma,\alpha} = \sum_{a \in V} W^2_{a,\alpha} Y^1_{a,\gamma} \quad (2r_T r_V N_v) \quad (11057)$$

$$\tau^2_{\gamma,\alpha} = \sum_{a \in V} W^2_{a,\alpha} Y^3_{a,\gamma} \quad (2r_T r_V N_v) \quad (11046)$$

$$\tau^3_{\gamma,\alpha,i} = \sum_{\delta \in A} Y^2_{i,\delta} Z_{\delta,\gamma} \tau^2_{\delta,\alpha} \quad (3r_T^2 r_V N_o) \quad (11058)$$

$$\tau^3_{\gamma,\alpha,i} = \sum_{\delta \in A} Z_{\gamma,\delta} Y^4_{i,\delta} \tau^2_{\delta,\alpha} \quad (3r_T^2 r_V N_o) \quad (11047)$$

$$\tau^4_{\gamma,\delta,\alpha,w} = \sum_{i \in O} {}^2D^2_{i,w} Y^{2,*}_{i,\delta} \tau^1_{\delta,\alpha,w} \tau^3_{\gamma,\alpha,i} \quad (4r_D r_T^2 r_V N_o) \quad (11059)$$

$$\tau^4_{\gamma,\delta,\alpha,w} = \sum_{i \in O} {}^2D^2_{i,w} Y^{2,*}_{i,\delta} \tau^1_{\delta,\alpha,w} \tau^3_{\gamma,\alpha,i} \quad (4r_D r_T^2 r_V N_o) \quad (11048)$$

$$\tau^5_{\alpha,i,j} = \sum_{\beta \in B} X_{\alpha,\beta} W^3_{i,\beta} W^4_{j,\beta} \quad (3r_V^2 N_o^2) \quad (11060)$$

$$\tau^5_{\alpha,i,j} = \sum_{\beta \in B} X_{\alpha,\beta} W^3_{i,\beta} W^4_{j,\beta} \quad (3r_V^2 N_o^2) \quad (11049)$$

$$\tau^6_{\gamma,\alpha,i} = \sum_{j \in O} Y^4_{j,\gamma} \tau^5_{\alpha,j,i} \quad (2r_T r_V N_o^2) \quad (11061)$$

$$\tau^6_{\gamma,\alpha,i} = \sum_{j \in O} Y^2_{j,\gamma} \tau^5_{\alpha,j,i} \quad (2r_T r_V N_o^2) \quad (11050)$$

$$\tau^7_{\gamma,\delta,w,i} = \sum_{\alpha \in B} \tau^6_{\gamma,\alpha,i} \tau^4_{\gamma,\delta,\alpha,w} \quad (2r_D r_T^2 r_V N_o) \quad (11062)$$

$$\tau^7_{\gamma,\delta,w,i} = \sum_{\alpha \in B} \tau^6_{\gamma,\alpha,i} \tau^4_{\gamma,\delta,\alpha,w} \quad (2r_D r_T^2 r_V N_o) \quad (11051)$$

$$\tau^8_{\gamma,\delta,i} = \sum_{\epsilon \in A} \sum_{w \in D} {}^2D^4_{i,w} \tau^0_{\epsilon,\delta,w} \tau^7_{\epsilon,\gamma,w,i} \quad (3r_D r_T^3 N_o) \quad (11063)$$

$${}^2R^4_{i,\gamma} \leftarrow - \sum_{\delta \in A} \frac{1}{2} Z^*_{\delta,\gamma} \tau^8_{\delta,\gamma,i} \quad (2r_T^2 N_o) \quad (11064)$$

Raw expression

$${}^2R^4_{j,\zeta} \leftarrow \sum_{\gamma \in A} \sum_{i \in O} \sum_{a \in V} \sum_{b \in V} \sum_{c \in V} \frac{1}{2} Y^{1,*}_{a,\gamma} Y^{2,*}_{i,\gamma} Z^*_{\gamma,\zeta} Y^{3,*}_{b,\zeta} f_{a,c} {}^2D^{a,i,b,j} {}^2T_{b,j,c,i} \quad (11065)$$

Factorized expression

$$\tau^0_{\gamma,\delta,w} = \sum_{a \in V} {}^2D^3_{a,w} Y^1_{a,\gamma} Y^{3,*}_{a,\delta} \quad (3r_D r_T^2 N_v) \quad (11066)$$

$$\tau^1_{\gamma,\alpha} = \sum_{i \in O} W^3_{i,\alpha} Y^2_{i,\gamma} \quad (2r_T r_V N_o) \quad (11067)$$

$$\tau^2_{\gamma,\alpha} = \sum_{a \in V} W^4_{a,\alpha} Y^3_{a,\gamma} \quad (2r_T r_V N_v) \quad (11068)$$

$$\tau^3_{\gamma,\alpha,i} = \sum_{\delta \in A} Z_{\gamma,\delta} Y^4_{i,\delta} \tau^2_{\delta,\alpha} \quad (3r_T^2 r_V N_o) \quad (11069)$$

$$\tau^4_{\gamma,\alpha,w} = \sum_{a \in V} {}^2D^1_{a,w} W^1_{a,\alpha} Y^{1,*}_{a,\gamma} \quad (3r_D r_T r_V N_v) \quad (11070)$$

$$\tau^5_{\gamma,\alpha,w} = \sum_{i \in O} {}^2D^2_{i,w} W^2_{i,\alpha} Y^{2,*}_{i,\gamma} \quad (3r_D r_T r_V N_o) \quad (11071)$$

$$\tau^6_{\gamma,\alpha,w} = \sum_{\beta \in B} X_{\beta,\alpha} \tau^4_{\gamma,\beta,w} \tau^5_{\gamma,\beta,w} \quad (3r_D r_T r_V^2) \quad (11072)$$

$$\tau^7_{\gamma,\alpha,w} = \sum_{\delta \in A} Z^*_{\delta,\gamma} \tau^6_{\delta,\alpha,w} \quad (2r_D r_T^2 r_V) \quad (11073)$$

$$\tau^8_{\gamma,\delta,w,i} = \sum_{\alpha \in B} \tau^1_{\gamma,\alpha} \tau^3_{\gamma,\alpha,i} \tau^7_{\delta,\alpha,w} \quad (3r_D r_T^2 r_V N_o) \quad (11074)$$

$$\tau^9_{\gamma,w,i} = \sum_{\delta \in A} \tau^0_{\delta,\gamma,w} \tau^8_{\delta,\gamma,w,i} \quad (2r_D r_T^2 N_o) \quad (11075)$$

$${}^2R^4_{i,\gamma} \leftarrow - \sum_{w \in D} \frac{1}{2} {}^2D^4_{i,w} \tau^9_{\gamma,w,i} \quad (2r_D r_T N_o) \quad (11076)$$

Raw expression

$${}^2R^4_{j,\zeta} \leftarrow \sum_{\gamma \in A} \sum_{i \in O} \sum_{a \in V} \sum_{b \in V} \sum_{c \in V} \frac{1}{2} Y^{1,*}_{a,\gamma} Y^{2,*}_{i,\gamma} Z^*_{\gamma,\zeta} Y^{3,*}_{b,\zeta} f_{a,c} {}^2D^{a,i,b,j} {}^2T_{c,i,b,j} \quad (11077)$$

Factorized expression

$$\tau^0_{\gamma,\delta,w} = \sum_{a \in V} {}^2D^3_{a,w} Y^3_{a,\gamma} Y^{3,*}_{a,\delta} \quad (3r_D r_T^2 N_v) \quad (11078)$$

$$\tau^1_{\gamma,\alpha} = \sum_{a \in V} W^4_{a,\alpha} Y^1_{a,\gamma} \quad (2r_T r_V N_v) \quad (11079)$$

$$\tau^2_{\gamma,\alpha,i} = \sum_{\delta \in A} Y^2_{i,\delta} Z_{\delta,\gamma} \tau^1_{\delta,\alpha} \quad (3r_T^2 r_V N_o) \quad (11080)$$

$$\tau^3_{\gamma,\alpha} = \sum_{i \in O} W^3_{i,\alpha} Y^4_{i,\gamma} \quad (2r_T r_V N_o) \quad (11081)$$

$$\tau^4_{\gamma,\alpha,w} = \sum_{a \in V} {}^2D^1_{a,w} W^1_{a,\alpha} Y^{1,*}_{a,\gamma} \quad (3r_D r_T r_V N_v) \quad (11082)$$

$$\tau^5_{\gamma,\alpha,w} = \sum_{i \in O} {}^2D^2_{i,w} W^2_{i,\alpha} Y^{2,*}_{i,\gamma} \quad (3r_D r_T r_V N_o) \quad (11083)$$

$$\tau^6_{\gamma,\alpha,w} = \sum_{\beta \in B} X_{\beta,\alpha} \tau^4_{\gamma,\beta,w} \tau^5_{\gamma,\beta,w} \quad (3r_D r_T r_V^2) \quad (11084)$$

$$\tau^7_{\gamma,\alpha,w} = \sum_{\delta \in A} Z^*_{\delta,\gamma} \tau^6_{\delta,\alpha,w} \quad (2r_D r_T^2 r_V) \quad (11085)$$

$$\tau^8_{\gamma,\delta,w,i} = \sum_{\alpha \in B} \tau^3_{\gamma,\alpha} \tau^2_{\gamma,\alpha,i} \tau^7_{\delta,\alpha,w} \quad (3r_D r_T^2 r_V N_o) \quad (11086)$$

$$\tau^9_{\gamma,w,i} = \sum_{\delta \in A} \tau^0_{\delta,\gamma,w} \tau^8_{\delta,\gamma,w,i} \quad (2r_D r_T^2 N_o) \quad (11087)$$

$${}^2R^4_{i,\gamma} \leftarrow - \sum_{w \in D} \frac{1}{2} {}^2D^4_{i,w} \tau^9_{\gamma,w,i} \quad (2r_D r_T N_o) \quad (11088)$$

Raw expression

$${}^2R^4_{j,\zeta} \leftarrow \sum_{\gamma \in A} \sum_{i \in O} \sum_{a \in V} \sum_{b \in V} \sum_{c \in V} \frac{1}{2} Y^{1,*}_{a,\gamma} Y^{2,*}_{i,\gamma} Z^*_{\gamma,\zeta} Y^{3,*}_{b,\zeta} f_{b,c} {}^2D^{a,i,b,j} {}^2T_{a,i,c,j} \quad (11089)$$

Factorized expression

$$\tau^0_{\gamma,\alpha,w} = \sum_{a \in V} {}^2D^3_{a,w} W^1_{a,\alpha} Y^{3,*}_{a,\gamma} \quad (3r_D r_T r_V N_v) \quad (11090)$$

$$\tau^1_{\gamma,\alpha} = \sum_{a \in V} W^2_{a,\alpha} Y^3_{a,\gamma} \quad (2r_T r_V N_v) \quad (11091)$$

$$\tau^2_{\gamma,\alpha,i} = \sum_{\delta \in A} Z_{\gamma,\delta} Y^4_{i,\delta} \tau^1_{\delta,\alpha} \quad (3r_T^2 r_V N_o) \quad (11092)$$

$$\tau^3_{\gamma,\delta,w} = \sum_{a \in V} {}^2D^1_{a,w} Y^1_{a,\gamma} Y^{1,*}_{a,\delta} \quad (3r_D r_T^2 N_v) \quad (11093)$$

$$\tau^4_{\gamma,\delta,w,i} = \sum_{\epsilon \in A} {}^2D^2_{i,w} Y^{2,*}_{i,\epsilon} Z^*_{\epsilon,\delta} \tau^3_{\gamma,\epsilon,w} \quad (4r_D r_T^3 N_o) \quad (11094)$$

$$\tau^5_{\alpha,i,j} = \sum_{\beta \in B} X_{\alpha,\beta} W^3_{i,\beta} W^4_{j,\beta} \quad (3r_V^2 N_o^2) \quad (11095)$$

$$\tau^6_{\gamma,\alpha,i} = \sum_{j \in O} Y^2_{j,\gamma} \tau^5_{\alpha,j,i} \quad (2r_T r_V N_o^2) \quad (11096)$$

$$\tau^7_{\gamma,\delta,\alpha,w} = \sum_{i \in O} \tau^6_{\gamma,\alpha,i} \tau^4_{\gamma,\delta,w,i} \quad (2r_D r_T^2 r_V N_o) \quad (11097)$$

$$\tau^8_{\gamma,\alpha,w,i} = \sum_{\delta \in A} \tau^2_{\delta,\alpha,i} \tau^7_{\delta,\gamma,\alpha,w} \quad (2r_D r_T^2 r_V N_o) \quad (11098)$$

$$\tau^9_{\gamma,w,i} = \sum_{\alpha \in B} \tau^0_{\gamma,\alpha,w} \tau^8_{\gamma,\alpha,w,i} \quad (2r_D r_T r_V N_o) \quad (11099)$$

$${}^2R^4_{i,\gamma} \leftarrow - \sum_{w \in D} \frac{1}{2} {}^2D^4_{i,w} \tau^9_{\gamma,w,i} \quad (2r_D r_T N_o) \quad (11100)$$

Raw expression

$${}^2R^4_{j,\zeta} \leftarrow \sum_{\gamma \in A} \sum_{i \in O} \sum_{a \in V} \sum_{b \in V} \sum_{c \in V} \frac{1}{2} Y^{1,*}_{a,\gamma} Y^{2,*}_{i,\gamma} Z^*_{\gamma,\zeta} Y^{3,*}_{b,\zeta} f_{b,c} {}^2D^{a,i,b,j} {}^2T_{c,j,a,i} \quad (11101)$$

Factorized expression

$$\tau^0_{\gamma,\alpha,w} = \sum_{a \in V} {}^2D^3_{a,w} W^1_{a,\alpha} Y^{3,*}_{a,\gamma} \quad (3r_D r_T r_V N_v) \quad (11102)$$

$$\tau^1_{\gamma,\delta,w} = \sum_{a \in V} {}^2D^1_{a,w} Y^3_{a,\gamma} Y^{1,*}_{a,\delta} \quad (3r_D r_T^2 N_v) \quad (11103)$$

$$\tau^2_{\gamma,\delta,w,i} = \sum_{\epsilon \in A} {}^2D^2_{i,w} Y^{2,*}_{i,\epsilon} Z^*_{\epsilon,\delta} \tau^1_{\gamma,\epsilon,w} \quad (4r_D r_T^3 N_o) \quad (11104)$$

$$\tau^3_{\alpha,i,j} = \sum_{\beta \in B} X_{\alpha,\beta} W^3_{i,\beta} W^4_{j,\beta} \quad (3r_V^2 N_o^2) \quad (11105)$$

$$\tau^4_{\gamma,\alpha,i} = \sum_{j \in O} Y^4_{j,\gamma} \tau^3_{\alpha,j,i} \quad (2r_T r_V N_o^2) \quad (11106)$$

$$\tau^5_{\gamma,\delta,\alpha,w} = \sum_{i \in O} \tau^4_{\gamma,\alpha,i} \tau^2_{\gamma,\delta,w,i} \quad (2r_D r_T^2 r_V N_o) \quad (11107)$$

$$\tau^6_{\gamma,\alpha} = \sum_{a \in V} W^2_{a,\alpha} Y^1_{a,\gamma} \quad (2r_T r_V N_v) \quad (11108)$$

$$\tau^7_{\gamma,\alpha,i} = \sum_{\delta \in A} Y^2_{i,\delta} Z_{\delta,\gamma} \tau^6_{\delta,\alpha} \quad (3r_T^2 r_V N_o) \quad (11109)$$

$$\tau^8_{\gamma,\alpha,w,i} = \sum_{\delta \in A} \tau^7_{\delta,\alpha,i} \tau^5_{\delta,\gamma,\alpha,w} \quad (2r_D r_T^2 r_V N_o) \quad (11110)$$

$$\tau^9_{\gamma,w,i} = \sum_{\alpha \in B} \tau^0_{\gamma,\alpha,w} \tau^8_{\gamma,\alpha,w,i} \quad (2r_D r_T r_V N_o) \quad (11111)$$

$${}^2R^4_{i,\gamma} \leftarrow - \sum_{w \in D} \frac{1}{2} {}^2D^4_{i,w} \tau^9_{\gamma,w,i} \quad (2r_D r_T N_o) \quad (11112)$$

Raw expression

$${}^2R^4_{j,\zeta} \leftarrow \sum_{\gamma \in A} \sum_{i \in O} \sum_{k \in O} \sum_{a \in V} \sum_{b \in V} \sum_{c \in V} Y^{1,*}_{a,\gamma} Y^{2,*}_{i,\gamma} Z^*_{\gamma,\zeta} Y^{3,*}_{b,\zeta} {}^2D^{a,i,b,j} {}^2T_{a,i,c,k} V_{b,j,k,c} \quad (11113)$$

Factorized expression

$$\tau^0_{\alpha,i,j} = \sum_{\beta \in B} X_{\alpha,\beta} W^3_{i,\beta} W^4_{j,\beta} \quad (3r_V^2 N_o^2) \quad (11114)$$

$$\tau^1_{\gamma,\alpha,i} = \sum_{j \in O} Y^4_{j,\gamma} \tau^0_{\alpha,j,i} \quad (2r_T r_V N_o^2) \quad (11115)$$

$$\tau^2_{\gamma,\alpha} = \sum_{a \in V} W^2_{a,\alpha} Y^3_{a,\gamma} \quad (2r_T r_V N_v) \quad (11116)$$

$$\tau^3_{\gamma,i,a} = \sum_{\alpha \in B} W^1_{a,\alpha} \tau^2_{\gamma,\alpha} \tau^1_{\gamma,\alpha,i} \quad (3r_T r_V N_o N_v) \quad (11117)$$

$$\tau^4_{\gamma,\delta,w} = \sum_{a \in V} {}^2D^1_{a,w} Y^1_{a,\gamma} Y^{1,*}_{a,\delta} \quad (3r_D r_T^2 N_v) \quad (11118)$$

$$\tau^5_{\gamma,\delta,w} = \sum_{i \in O} {}^2D^2_{i,w} Y^2_{i,\gamma} Y^{2,*}_{i,\delta} \quad (3r_D r_T^2 N_o) \quad (11119)$$

$$\tau^6_{\gamma,\delta,w} = \sum_{\epsilon \in A} Z^*_{\epsilon,\delta} \tau^4_{\gamma,\epsilon,w} \tau^5_{\gamma,\epsilon,w} \quad (3r_D r_T^3) \quad (11120)$$

$$\tau^7_{\gamma,\delta,w} = \sum_{\epsilon \in A} Z_{\epsilon,\gamma} \tau^6_{\epsilon,\delta,w} \quad (2r_D r_T^3) \quad (11121)$$

$$\tau^8_{\gamma,i,a} = \sum_{\delta \in A} \sum_{w \in D} {}^2D^3_{a,w} {}^2D^4_{i,w} \tau^3_{\delta,i,a} \tau^7_{\delta,\gamma,w} \quad (4r_D r_T^2 N_o N_v) \quad (11122)$$

$${}^2R^4_{i,\gamma} \leftarrow - \sum_{a \in V} \frac{1}{2} Y^{3,*}_{a,\gamma} \tau^8_{\gamma,i,a} \quad (2r_T N_o N_v) \quad (11123)$$

Raw expression

$${}^2R^4_{j,\zeta} \leftarrow \sum_{\gamma \in A} \sum_{i \in O} \sum_{k \in O} \sum_{a \in V} \sum_{b \in V} \sum_{c \in V} Y^{1,*}_{a,\gamma} Y^{2,*}_{i,\gamma} Z^*_{\gamma,\zeta} Y^{3,*}_{b,\zeta} {}^2D^{a,i,b,j} {}^2T_{b,j,c,k} V_{a,i,k,c} \quad (11124)$$

Factorized expression

$$\tau^0_{\alpha,i,j} = \sum_{\beta \in B} X_{\alpha,\beta} W^3_{i,\beta} W^4_{j,\beta} \quad (3r_V^2 N_o^2) \quad (11125)$$

$$\tau^1_{\gamma,\alpha,i} = \sum_{j \in O} Y^2_{j,\gamma} \tau^0_{\alpha,j,i} \quad (2r_T r_V N_o^2) \quad (11126)$$

$$\tau^2_{\gamma,\alpha} = \sum_{a \in V} W^2_{a,\alpha} Y^1_{a,\gamma} \quad (2r_T r_V N_v) \quad (11127)$$

$$\tau^3_{\gamma,i,a} = \sum_{\alpha \in B} W^1_{a,\alpha} \tau^2_{\gamma,\alpha} \tau^1_{\gamma,\alpha,i} \quad (3r_T r_V N_o N_v) \quad (11128)$$

$$\tau^4_{\gamma,\delta,w} = \sum_{a \in V} {}^2D^1_{a,w} Y^3_{a,\gamma} Y^{1,*}_{a,\delta} \quad (3r_D r_T^2 N_v) \quad (11129)$$

$$\tau^5_{\gamma,\delta,w} = \sum_{i \in O} {}^2D^2_{i,w} Y^4_{i,\gamma} Y^{2,*}_{i,\delta} \quad (3r_D r_T^2 N_o) \quad (11130)$$

$$\tau^6_{\gamma,\delta,w} = \sum_{\epsilon \in A} Z^*_{\epsilon,\delta} \tau^4_{\gamma,\epsilon,w} \tau^5_{\gamma,\epsilon,w} \quad (3r_D r_T^3) \quad (11131)$$

$$\tau^7_{\gamma,\delta,w} = \sum_{\epsilon \in A} Z_{\gamma,\epsilon} \tau^6_{\epsilon,\delta,w} \quad (2r_D r_T^3) \quad (11132)$$

$$\tau^8_{\gamma,i,a} = \sum_{\delta \in A} \sum_{w \in D} {}^2D^3_{a,w} {}^2D^4_{i,w} \tau^3_{\delta,i,a} \tau^7_{\delta,\gamma,w} \quad (4r_D r_T^2 N_o N_v) \quad (11133)$$

$${}^2R^4_{i,\gamma} \leftarrow - \sum_{a \in V} \frac{1}{2} Y^{3,*}_{a,\gamma} \tau^8_{\gamma,i,a} \quad (2r_T N_o N_v) \quad (11134)$$

Raw expression

$${}^2R^4_{j,\zeta} \leftarrow \sum_{\gamma \in A} \sum_{i \in O} \sum_{k \in O} \sum_{a \in V} \sum_{b \in V} \sum_{c \in V} Y^{1,*}_{a,\gamma} Y^{2,*}_{i,\gamma} Z^*_{\gamma,\zeta} Y^{3,*}_{b,\zeta} {}^2D^{a,i,b,j} {}^2T_{c,k,a,i} V_{b,j,k,c} \quad (11135)$$

Factorized expression

$$\tau^0_{\gamma,\alpha,w} = \sum_{a \in V} {}^2D^3_{a,w} W^1_{a,\alpha} Y^{3,*}_{a,\gamma} \quad (3r_D r_T r_V N_v) \quad (11136)$$

$$\tau^1_{\gamma,\delta,w} = \sum_{a \in V} {}^2D^1_{a,w} Y^1_{a,\gamma} Y^{1,*}_{a,\delta} \quad (3r_D r_T^2 N_v) \quad (11137)$$

$$\tau^2_{\gamma,\alpha} = \sum_{a \in V} W^4_{a,\alpha} Y^1_{a,\gamma} \quad (2r_T r_V N_v) \quad (11149)$$

$$\tau^2_{\gamma,\alpha} = \sum_{i \in O} W^3_{i,\alpha} Y^2_{i,\gamma} \quad (2r_T r_V N_o) \quad (11138)$$

$$\tau^3_{\gamma,\alpha,i} = \sum_{\delta \in A} Y^2_{i,\delta} Z_{\delta,\gamma} \tau^2_{\delta,\alpha} \quad (3r_T^2 r_V N_o) \quad (11150)$$

$$\tau^3_{\gamma,\alpha} = \sum_{a \in V} W^4_{a,\alpha} Y^3_{a,\gamma} \quad (2r_T r_V N_v) \quad (11139)$$

$$\tau^4_{\gamma,\alpha} = \sum_{i \in O} W^3_{i,\alpha} Y^4_{i,\gamma} \quad (2r_T r_V N_o) \quad (11151)$$

$$\tau^4_{\gamma,\alpha,i} = \sum_{\delta \in A} Z_{\gamma,\delta} Y^4_{i,\delta} \tau^3_{\delta,\alpha} \quad (3r_T^2 r_V N_o) \quad (11140)$$

$$\tau^5_{\gamma,\alpha,w} = \sum_{\delta \in A} \sum_{i \in O} {}^2D^2_{i,w} Y^{2,*}_{i,\gamma} \tau^4_{\delta,\alpha} \tau^1_{\delta,\gamma,w} \tau^3_{\delta,\alpha,i} \quad (5r_D r_T^2 r_V N_o) \quad (11152)$$

$$\tau^5_{\gamma,\alpha,w} = \sum_{\delta \in A} \sum_{i \in O} {}^2D^2_{i,w} Y^{2,*}_{i,\gamma} \tau^2_{\delta,\alpha} \tau^1_{\delta,\gamma,w} \tau^4_{\delta,\alpha,i} \quad (5r_D r_T^2 r_V N_o) \quad (11141)$$

$$\tau^6_{\gamma,\alpha,w} = \sum_{\beta \in B} X_{\alpha,\beta} \tau^5_{\gamma,\beta,w} \quad (2r_D r_T r_V^2) \quad (11153)$$

$$\tau^6_{\gamma,\alpha,w} = \sum_{\beta \in B} X_{\alpha,\beta} \tau^5_{\gamma,\beta,w} \quad (2r_D r_T r_V^2) \quad (11142)$$

$$\tau^7_{\gamma,\alpha,w} = \sum_{\delta \in A} Z^*_{\delta,\gamma} \tau^6_{\delta,\alpha,w} \quad (2r_D r_T^2 r_V) \quad (11154)$$

$$\tau^7_{\gamma,\alpha,w} = \sum_{\delta \in A} Z^*_{\delta,\gamma} \tau^6_{\delta,\alpha,w} \quad (2r_D r_T^2 r_V) \quad (11143)$$

$$\tau^8_{\gamma,w,i} = \sum_{\alpha \in B} W^2_{i,\alpha} \tau^0_{\gamma,\alpha,w} \tau^7_{\gamma,\alpha,w} \quad (3r_D r_T r_V N_o) \quad (11155)$$

$$\tau^8_{\gamma,w,i} = \sum_{\alpha \in B} W^2_{i,\alpha} \tau^0_{\gamma,\alpha,w} \tau^7_{\gamma,\alpha,w} \quad (3r_D r_T r_V N_o) \quad (11144)$$

$${}^2R^4_{i,\gamma} \leftarrow - \sum_{w \in D} \frac{1}{2} {}^2D^4_{i,w} \tau^8_{\gamma,w,i} \quad (2r_D r_T N_o) \quad (11156)$$

Raw expression

$${}^2R^4_{i,\gamma} \leftarrow - \sum_{w \in D} \frac{1}{2} {}^2D^4_{i,w} \tau^8_{\gamma,w,i} \quad (2r_D r_T N_o) \quad (11145)$$

$${}^2R^4_{j,\zeta} \leftarrow - \sum_{\gamma \in A} \sum_{i \in O} \sum_{k \in O} \sum_{a \in V} \sum_{b \in V} \sum_{c \in V} \frac{1}{2} Y^{1,*}_{a,\gamma} Y^{2,*}_{i,\gamma} Z^*_{\gamma,\zeta} Y^{3,*}_{b,\zeta} {}^2D^{a,i,b,j} {}^2T_{a,i,c,k} V_{b,c,k,j} \quad (11157)$$

Raw expression

$${}^2R^4_{j,\zeta} \leftarrow \sum_{\gamma \in A} \sum_{i \in O} \sum_{k \in O} \sum_{a \in V} \sum_{b \in V} \sum_{c \in V} Y^{1,*}_{a,\gamma} Y^{2,*}_{i,\gamma} Z^*_{\gamma,\zeta} Y^{3,*}_{b,\zeta} {}^2D^{a,i,b,j} {}^2T_{c,k,b,j} V_{a,i,k,c} \quad (11146)$$

Factorized expression

Factorized expression

$$\tau^0_{\gamma,\alpha,w} = \sum_{a \in V} {}^2D^3_{a,w} W^1_{a,\alpha} Y^{3,*}_{a,\gamma} \quad (3r_D r_T r_V N_v) \quad (11147)$$

$$\tau^1_{\gamma,\delta,w} = \sum_{a \in V} {}^2D^1_{a,w} Y^1_{a,\gamma} Y^{1,*}_{a,\delta} \quad (3r_D r_T^2 N_v) \quad (11159)$$

$$\tau^1_{\gamma,\delta,w} = \sum_{a \in V} {}^2D^1_{a,w} Y^3_{a,\gamma} Y^{1,*}_{a,\delta} \quad (3r_D r_T^2 N_v) \quad (11148)$$

$$\tau^2_{\gamma,\delta,w} = \sum_{i \in O} {}^2D^2_{i,w} Y^2_{i,\gamma} Y^{2,*}_{i,\delta} \quad (3r_D r_T^2 N_o) \quad (11160)$$

$$\tau^3_{\gamma,\delta,w} = \sum_{\epsilon \in A} Z^*_{\epsilon,\delta} \tau^1_{\gamma,\epsilon,w} \tau^2_{\gamma,\epsilon,w} \quad (3r_D r_T^3) \quad (11161)$$

$$\tau^4_{\gamma,\delta,w} = \sum_{\epsilon \in A} Z_{\epsilon,\gamma} \tau^3_{\epsilon,\delta,w} \quad (2r_D r_T^3) \quad (11162)$$

$$\tau^5_{\gamma,i} = \sum_{j \in O} Y^4_{j,\gamma} f_{j,i} \quad (2r_T N_o^2) \quad (11163)$$

$${}^2R^4_{i,\gamma} \leftarrow - \sum_{\delta \in A} \sum_{w \in D} \frac{1}{2} {}^2D^4_{i,w} \tau^5_{\delta,i} \tau^0_{\delta,\gamma,w} \tau^4_{\delta,\gamma,w} \quad (4r_D r_T^2 N_o) \quad (11164)$$

Raw expression

$${}^2R^4_{j,\zeta} \leftarrow - \sum_{\gamma \in A} \sum_{i \in O} \sum_{k \in O} \sum_{a \in V} \sum_{b \in V} \sum_{c \in V} \frac{1}{2} Y^{1,*}_{a,\gamma} Y^{2,*}_{i,\gamma} Z^*_{\gamma,\zeta} Y^{3,*}_{b,\zeta} {}^2D^{a,i,b,j} {}^2T_{a,k,c,i} V_{b,j,k,c} \quad (11165)$$

Factorized expression

$$\tau^0_{\gamma,\delta,w} = \sum_{a \in V} {}^2D^3_{a,w} Y^3_{a,\gamma} Y^{3,*}_{a,\delta} \quad (3r_D r_T^2 N_v) \quad (11166)$$

$$\tau^1_{\gamma,\delta,w} = \sum_{a \in V} {}^2D^1_{a,w} Y^1_{a,\gamma} Y^{1,*}_{a,\delta} \quad (3r_D r_T^2 N_v) \quad (11167)$$

$$\tau^2_{\gamma,i} = \sum_{j \in O} Y^2_{j,\gamma} f_{j,i} \quad (2r_T N_o^2) \quad (11168)$$

$$\tau^3_{\gamma,\delta,w} = \sum_{i \in O} {}^2D^2_{i,w} Y^{2,*}_{i,\delta} \tau^2_{\gamma,i} \quad (3r_D r_T^2 N_o) \quad (11169)$$

$$\tau^4_{\gamma,\delta,w} = \sum_{\epsilon \in A} Z^*_{\epsilon,\delta} \tau^1_{\gamma,\epsilon,w} \tau^3_{\gamma,\epsilon,w} \quad (3r_D r_T^3) \quad (11170)$$

$$\tau^5_{\gamma,\delta,w} = \sum_{\epsilon \in A} Z_{\epsilon,\gamma} \tau^4_{\epsilon,\delta,w} \quad (2r_D r_T^3) \quad (11171)$$

$${}^2R^4_{i,\gamma} \leftarrow - \sum_{\delta \in A} \sum_{w \in D} \frac{1}{2} {}^2D^4_{i,w} Y^4_{i,\delta} \tau^0_{\delta,\gamma,w} \tau^5_{\delta,\gamma,w} \quad (4r_D r_T^2 N_o) \quad (11172)$$

Raw expression

$${}^2R^4_{j,\zeta} \leftarrow - \sum_{\gamma \in A} \sum_{i \in O} \sum_{k \in O} \sum_{a \in V} \sum_{b \in V} \sum_{c \in V} \frac{1}{2} Y^{1,*}_{a,\gamma} Y^{2,*}_{i,\gamma} Z^*_{\gamma,\zeta} Y^{3,*}_{b,\zeta} {}^2D^{a,i,b,j} {}^2T_{a,k,c,j} V_{b,c,k,i} \quad (11173)$$

Factorized expression

$$\tau^0_{\gamma,\delta,w} = \sum_{a \in V} {}^2D^3_{a,w} Y^1_{a,\gamma} Y^{3,*}_{a,\delta} \quad (3r_D r_T^2 N_v) \quad (11174)$$

$$\tau^1_{\gamma,\delta,w} = \sum_{a \in V} {}^2D^1_{a,w} Y^3_{a,\gamma} Y^{1,*}_{a,\delta} \quad (3r_D r_T^2 N_v) \quad (11175)$$

$$\tau^2_{\gamma,i} = \sum_{j \in O} Y^4_{j,\gamma} f_{j,i} \quad (2r_T N_o^2) \quad (11176)$$

$$\tau^3_{\gamma,\delta,w} = \sum_{i \in O} {}^2D^2_{i,w} Y^{2,*}_{i,\delta} \tau^2_{\gamma,i} \quad (3r_D r_T^2 N_o) \quad (11177)$$

$$\tau^4_{\gamma,\delta,w} = \sum_{\epsilon \in A} Z^*_{\epsilon,\delta} \tau^1_{\gamma,\epsilon,w} \tau^3_{\gamma,\epsilon,w} \quad (3r_D r_T^3) \quad (11178)$$

$$\tau^5_{\gamma,\delta,w} = \sum_{\epsilon \in A} Z_{\gamma,\epsilon} \tau^4_{\epsilon,\delta,w} \quad (2r_D r_T^3) \quad (11179)$$

$${}^2R^4_{i,\gamma} \leftarrow - \sum_{\delta \in A} \sum_{w \in D} \frac{1}{2} {}^2D^4_{i,w} Y^2_{i,\delta} \tau^0_{\delta,\gamma,w} \tau^5_{\delta,\gamma,w} \quad (4r_D r_T^2 N_o) \quad (11180)$$

Raw expression

$${}^2R^4_{j,\zeta} \leftarrow - \sum_{\gamma \in A} \sum_{i \in O} \sum_{k \in O} \sum_{a \in V} \sum_{b \in V} \sum_{c \in V} \frac{1}{2} Y^{1,*}_{a,\gamma} Y^{2,*}_{i,\gamma} Z^*_{\gamma,\zeta} Y^{3,*}_{b,\zeta} {}^2D^{a,i,b,j} {}^2T_{b,j,c,k} V_{a,c,k,i} \quad (11181)$$

Factorized expression

$$\tau^0_{\gamma,\delta,w} = \sum_{a \in V} {}^2D^3_{a,w} Y^1_{a,\gamma} Y^{3,*}_{a,\delta} \quad (3r_D r_T^2 N_v) \quad (11182)$$

$$\tau^1_{\gamma,\delta,w} = \sum_{a \in V} {}^2D^1_{a,w} Y^3_{a,\gamma} Y^{1,*}_{a,\delta} \quad (3r_D r_T^2 N_v) \quad (11183)$$



$$\tau_{\gamma,\delta,w}^2 = \sum_{i \in O} {}^2D_{i,w}^2 Y_{i,\gamma}^4 Y_{i,\delta}^{2,*} \quad (3r_D r_T^2 N_o) \quad (11184)$$

$$\tau_{\gamma,\alpha,i}^6 = \sum_{j \in O} Y_{j,\gamma}^4 \tau_{\alpha,j,i}^5 \quad (2r_T r_V N_o^2) \quad (11196)$$

$$\tau_{\gamma,\delta,w}^3 = \sum_{\epsilon \in A} Z_{\epsilon,\delta}^* \tau_{\gamma,\epsilon,w}^1 \tau_{\gamma,\epsilon,w}^2 \quad (3r_D r_T^3) \quad (11185)$$

$$\tau_{\gamma,\delta,w,i}^7 = \sum_{\alpha \in B} \tau_{\gamma,\alpha,i}^6 \tau_{\gamma,\delta,\alpha,w}^4 \quad (2r_D r_T^2 r_V N_o) \quad (11197)$$

$$\tau_{\gamma,\delta,w}^4 = \sum_{\epsilon \in A} Z_{\gamma,\epsilon} \tau_{\epsilon,\delta,w}^3 \quad (2r_D r_T^3) \quad (11186)$$

$$\tau_{\gamma,\delta,i}^8 = \sum_{\epsilon \in A} \sum_{w \in D} {}^2D_{i,w}^4 \tau_{\epsilon,\delta,w}^0 \tau_{\epsilon,\gamma,w,i}^7 \quad (3r_D r_T^3 N_o) \quad (11198)$$

$$\tau_{\gamma,i}^5 = \sum_{j \in O} Y_{j,\gamma}^2 f_{j,i} \quad (2r_T N_o^2) \quad (11187)$$

$${}^2R_{i,\gamma}^4 \leftarrow \sum_{\delta \in A} \frac{1}{2} Z_{\delta,\gamma}^* \tau_{\delta,\gamma,i}^8 \quad (2r_T^2 N_o) \quad (11199)$$

$${}^2R_{i,\gamma}^4 \leftarrow - \sum_{\delta \in A} \sum_{w \in D} \frac{1}{2} {}^2D_{i,w}^4 \tau_{\delta,i}^5 \tau_{\delta,\gamma,w}^0 \tau_{\delta,\gamma,w}^4 \quad (4r_D r_T^2 N_o) \quad (11188)$$

Raw expression

$${}^2R_{j,\zeta}^4 \leftarrow - \sum_{\gamma \in A} \sum_{i \in O} \sum_{k \in O} \sum_{a \in V} \sum_{b \in V} \sum_{c \in V} \frac{1}{2} Y_{a,\gamma}^{1,*} Y_{i,\gamma}^{2,*} Z_{\gamma,\zeta}^* Y_{b,\zeta}^{3,*} {}^2D_{a,i,b,j} {}^2T_{b,k,c,i} V_{a,c,k,j} \quad (11189)$$

Factorized expression

$$\tau_{\gamma,\delta,w}^0 = \sum_{a \in V} {}^2D_{a,w}^3 Y_{a,\gamma}^3 Y_{a,\delta}^{3,*} \quad (3r_D r_T^2 N_v) \quad (11190)$$

Raw expression

$${}^2R_{j,\zeta}^4 \leftarrow - \sum_{\gamma \in A} \sum_{i \in O} \sum_{k \in O} \sum_{a \in V} \sum_{b \in V} \sum_{c \in V} \frac{1}{2} Y_{a,\gamma}^{1,*} Y_{i,\gamma}^{2,*} Z_{\gamma,\zeta}^* Y_{b,\zeta}^{3,*} {}^2D_{a,i,b,j} {}^2T_{b,k,c,j} V_{a,i,k,c} \quad (11200)$$

Factorized expression

$$\tau_{\gamma,\delta,w}^0 = \sum_{a \in V} {}^2D_{a,w}^3 Y_{a,\gamma}^1 Y_{a,\delta}^{3,*} \quad (3r_D r_T^2 N_v) \quad (11201)$$

$$\tau_{\gamma,\alpha,w}^1 = \sum_{i \in O} {}^2D_{i,w}^2 W_{i,\alpha}^2 Y_{i,\gamma}^{2,*} \quad (3r_D r_T r_V N_o) \quad (11191)$$

$$\tau_{\gamma,\alpha,w}^1 = \sum_{i \in O} {}^2D_{i,w}^2 W_{i,\alpha}^2 Y_{i,\gamma}^{2,*} \quad (3r_D r_T r_V N_o) \quad (11202)$$

$$\tau_{\gamma,\delta,w}^2 = \sum_{a \in V} {}^2D_{a,w}^1 Y_{a,\gamma}^1 Y_{a,\delta}^{1,*} \quad (3r_D r_T^2 N_v) \quad (11192)$$

$$\tau_{\gamma,\delta,w}^2 = \sum_{a \in V} {}^2D_{a,w}^1 Y_{a,\gamma}^3 Y_{a,\delta}^{1,*} \quad (3r_D r_T^2 N_v) \quad (11203)$$

$$\tau_{\gamma,\delta,w,i}^3 = \sum_{\epsilon \in A} Y_{i,\epsilon}^2 Z_{\epsilon,\gamma} \tau_{\epsilon,\delta,w}^2 \quad (3r_D r_T^3 N_o) \quad (11193)$$

$$\tau_{\gamma,\delta,w,i}^3 = \sum_{\epsilon \in A} Z_{\gamma,\epsilon} Y_{i,\epsilon}^4 \tau_{\epsilon,\delta,w}^2 \quad (3r_D r_T^3 N_o) \quad (11204)$$

$$\tau_{\gamma,\delta,\alpha,w}^4 = \sum_{i \in O} W_{i,\alpha}^1 \tau_{\delta,\alpha,w}^1 \tau_{\gamma,\delta,w,i}^3 \quad (3r_D r_T^2 r_V N_o) \quad (11194)$$

$$\tau_{\gamma,\delta,\alpha,w}^4 = \sum_{i \in O} W_{i,\alpha}^1 \tau_{\delta,\alpha,w}^1 \tau_{\gamma,\delta,w,i}^3 \quad (3r_D r_T^2 r_V N_o) \quad (11205)$$

$$\tau_{\alpha,i,j}^5 = \sum_{\beta \in B} X_{\alpha,\beta} W_{i,\beta}^3 W_{j,\beta}^4 \quad (3r_V^2 N_o^2) \quad (11195)$$

$$\tau_{\alpha,i,j}^5 = \sum_{\beta \in B} X_{\alpha,\beta} W_{i,\beta}^3 W_{j,\beta}^4 \quad (3r_V^2 N_o^2) \quad (11206)$$

$$\tau_{\gamma,\alpha,i}^6 = \sum_{j \in O} Y_{j,\gamma}^2 \tau_{\alpha,j,i}^5 \quad (2r_T r_V N_o^2) \quad (11207)$$

$$\tau_{\gamma,\delta,w,i}^7 = \sum_{\alpha \in B} \tau_{\gamma,\alpha,i}^6 \tau_{\gamma,\delta,\alpha,w}^4 \quad (2r_D r_T^2 r_V N_o) \quad (11208)$$

$$\tau_{\gamma,\delta,i}^8 = \sum_{\epsilon \in A} \sum_{w \in D} {}^2D_{i,w}^4 \tau_{\epsilon,\delta,w}^0 \tau_{\epsilon,\gamma,w,i}^7 \quad (3r_D r_T^3 N_o) \quad (11209)$$

$${}^2R_{i,\gamma}^4 \leftarrow \sum_{\delta \in A} \frac{1}{2} Z_{\delta,\gamma}^* \tau_{\delta,\gamma,i}^8 \quad (2r_T^2 N_o) \quad (11210)$$

Raw expression

$${}^2R_{j,\zeta}^4 \leftarrow - \sum_{\gamma \in A} \sum_{i \in O} \sum_{k \in O} \sum_{a \in V} \sum_{b \in V} \sum_{c \in V} \frac{1}{2} Y_{a,\gamma}^{1,*} Y_{i,\gamma}^{2,*} Z_{\gamma,\zeta}^* Y_{b,\zeta}^{3,*} {}^2D_{a,i,b,j} {}^2T_{c,i,a,k} V_{b,j,k,c} \quad (11211)$$

Factorized expression

$$\tau_{\gamma,a}^0 = \sum_{b \in V} Y_{b,\gamma}^3 f_{a,b} \quad (2r_T N_v^2) \quad (11212)$$

$$\tau_{\gamma,\delta,w}^1 = \sum_{a \in V} {}^2D_{a,w}^3 Y_{a,\delta}^{3,*} \tau_{\gamma,a}^0 \quad (3r_D r_T^2 N_v) \quad (11213)$$

$$\tau_{\gamma,\delta,w}^2 = \sum_{a \in V} {}^2D_{a,w}^1 Y_{a,\gamma}^1 Y_{a,\delta}^{1,*} \quad (3r_D r_T^2 N_v) \quad (11214)$$

$$\tau_{\gamma,\delta,w}^3 = \sum_{i \in O} {}^2D_{i,w}^2 Y_{i,\gamma}^2 Y_{i,\delta}^{2,*} \quad (3r_D r_T^2 N_o) \quad (11215)$$

$$\tau_{\gamma,\delta,w}^4 = \sum_{\epsilon \in A} Z_{\epsilon,\delta}^* \tau_{\gamma,\epsilon,w}^2 \tau_{\gamma,\epsilon,w}^3 \quad (3r_D r_T^3) \quad (11216)$$

$$\tau_{\gamma,\delta,w}^5 = \sum_{\epsilon \in A} Z_{\epsilon,\gamma} \tau_{\epsilon,\delta,w}^4 \quad (2r_D r_T^3) \quad (11217)$$

$${}^2R_{i,\gamma}^4 \leftarrow \sum_{\delta \in A} \sum_{w \in D} \frac{1}{2} {}^2D_{i,w}^4 Y_{i,\delta}^4 \tau_{\delta,\gamma,w}^1 \tau_{\delta,\gamma,w}^5 \quad (4r_D r_T^2 N_o) \quad (11218)$$

Raw expression

$${}^2R_{j,\zeta}^4 \leftarrow - \sum_{\gamma \in A} \sum_{i \in O} \sum_{k \in O} \sum_{a \in V} \sum_{b \in V} \sum_{c \in V} \frac{1}{2} Y_{a,\gamma}^{1,*} Y_{i,\gamma}^{2,*} Z_{\gamma,\zeta}^* Y_{b,\zeta}^{3,*} {}^2D_{a,i,b,j} {}^2T_{c,i,b,k} V_{a,c,k,j} \quad (11219)$$

Factorized expression

$$\tau_{\gamma,\delta,w}^0 = \sum_{a \in V} {}^2D_{a,w}^3 Y_{a,\gamma}^1 Y_{a,\delta}^{3,*} \quad (3r_D r_T^2 N_v) \quad (11220)$$

$$\tau_{\gamma,\delta,w}^1 = \sum_{i \in O} {}^2D_{i,w}^2 Y_{i,\gamma}^4 Y_{i,\delta}^{2,*} \quad (3r_D r_T^2 N_o) \quad (11221)$$

$$\tau_{\gamma,a}^2 = \sum_{b \in V} Y_{b,\gamma}^3 f_{a,b} \quad (2r_T N_v^2) \quad (11222)$$

$$\tau_{\gamma,\delta,w}^3 = \sum_{a \in V} {}^2D_{a,w}^1 Y_{a,\delta}^{1,*} \tau_{\gamma,a}^2 \quad (3r_D r_T^2 N_v) \quad (11223)$$

$$\tau_{\gamma,\delta,w}^4 = \sum_{\epsilon \in A} Z_{\epsilon,\delta}^* \tau_{\gamma,\epsilon,w}^1 \tau_{\gamma,\epsilon,w}^3 \quad (3r_D r_T^3) \quad (11224)$$

$$\tau_{\gamma,\delta,w}^5 = \sum_{\epsilon \in A} Z_{\gamma,\epsilon} \tau_{\epsilon,\delta,w}^4 \quad (2r_D r_T^3) \quad (11225)$$

$${}^2R_{i,\gamma}^4 \leftarrow \sum_{\delta \in A} \sum_{w \in D} \frac{1}{2} {}^2D_{i,w}^4 Y_{i,\delta}^2 \tau_{\delta,\gamma,w}^0 \tau_{\delta,\gamma,w}^5 \quad (4r_D r_T^2 N_o) \quad (11226)$$

Raw expression

$${}^2R_{j,\zeta}^4 \leftarrow - \sum_{\gamma \in A} \sum_{i \in O} \sum_{k \in O} \sum_{a \in V} \sum_{b \in V} \sum_{c \in V} \frac{1}{2} Y_{a,\gamma}^{1,*} Y_{i,\gamma}^{2,*} Z_{\gamma,\zeta}^* Y_{b,\zeta}^{3,*} {}^2D_{a,i,b,j} {}^2T_{c,j,a,k} V_{b,c,k,i} \quad (11227)$$

Factorized expression

$$\tau_{\gamma,\delta,w}^0 = \sum_{a \in V} {}^2D_{a,w}^3 Y_{a,\gamma}^3 Y_{a,\delta}^{3,*} \quad (3r_D r_T^2 N_v) \quad (11228)$$

$$\tau_{\gamma,\delta,w}^1 = \sum_{i \in O} {}^2D_{i,w}^2 Y_{i,\gamma}^2 Y_{i,\delta}^{2,*} \quad (3r_D r_T^2 N_o) \quad (11229)$$

$$\tau_{\gamma,a}^2 = \sum_{b \in V} Y_{b,\gamma}^1 f_{a,b} \quad (2r_T N_v^2) \quad (11230)$$

$$\tau^3_{\gamma,\delta,w} = \sum_{a \in V} {}^2D^1_{a,w} Y^{1,*}_{a,\delta} \tau^2_{\gamma,a} \quad (3r_D r_T^2 N_v) \quad (11231)$$

$$\tau^4_{\gamma,\delta,w} = \sum_{\epsilon \in A} Z^*_{\epsilon,\delta} \tau^1_{\gamma,\epsilon,w} \tau^3_{\gamma,\epsilon,w} \quad (3r_D r_T^3) \quad (11232)$$

$$\tau^5_{\gamma,\delta,w} = \sum_{\epsilon \in A} Z_{\epsilon,\gamma} \tau^4_{\epsilon,\delta,w} \quad (2r_D r_T^3) \quad (11233)$$

$${}^2R^4_{i,\gamma} \leftarrow \sum_{\delta \in A} \sum_{w \in D} \frac{1}{2} {}^2D^4_{i,w} Y^4_{i,\delta} \tau^0_{\delta,\gamma,w} \tau^5_{\delta,\gamma,w} \quad (4r_D r_T^2 N_o) \quad (11234)$$

Raw expression

$${}^2R^4_{j,\zeta} \leftarrow - \sum_{\gamma \in A} \sum_{i \in O} \sum_{k \in O} \sum_{a \in V} \sum_{b \in V} \sum_{c \in V} \frac{1}{2} Y^{1,*}_{a,\gamma} Y^{2,*}_{i,\gamma} Z^*_{\gamma,\zeta} Y^{3,*}_{b,\zeta} {}^2D^{a,i,b,j} {}^2T_{c,j,b,k} V_{a,i,k,c} \quad (11235)$$

Factorized expression

$$\tau^0_{\gamma,a} = \sum_{b \in V} Y^1_{b,\gamma} f_{a,b} \quad (2r_T N_v^2) \quad (11236)$$

$$\tau^1_{\gamma,\delta,w} = \sum_{a \in V} {}^2D^3_{a,w} Y^{3,*}_{a,\delta} \tau^0_{\gamma,a} \quad (3r_D r_T^2 N_v) \quad (11237)$$

$$\tau^2_{\gamma,\delta,w} = \sum_{a \in V} {}^2D^1_{a,w} Y^3_{a,\gamma} Y^{1,*}_{a,\delta} \quad (3r_D r_T^2 N_v) \quad (11238)$$

$$\tau^3_{\gamma,\delta,w} = \sum_{i \in O} {}^2D^2_{i,w} Y^4_{i,\gamma} Y^{2,*}_{i,\delta} \quad (3r_D r_T^2 N_o) \quad (11239)$$

$$\tau^4_{\gamma,\delta,w} = \sum_{\epsilon \in A} Z^*_{\epsilon,\delta} \tau^2_{\gamma,\epsilon,w} \tau^3_{\gamma,\epsilon,w} \quad (3r_D r_T^3) \quad (11240)$$

$$\tau^5_{\gamma,\delta,w} = \sum_{\epsilon \in A} Z_{\gamma,\epsilon} \tau^4_{\epsilon,\delta,w} \quad (2r_D r_T^3) \quad (11241)$$

$${}^2R^4_{i,\gamma} \leftarrow \sum_{\delta \in A} \sum_{w \in D} \frac{1}{2} {}^2D^4_{i,w} Y^2_{i,\delta} \tau^1_{\delta,\gamma,w} \tau^5_{\delta,\gamma,w} \quad (4r_D r_T^2 N_o) \quad (11242)$$

Raw expression

$${}^2R^4_{j,\zeta} \leftarrow - \sum_{\gamma \in A} \sum_{i \in O} \sum_{k \in O} \sum_{a \in V} \sum_{b \in V} \sum_{c \in V} \frac{1}{2} Y^{1,*}_{a,\gamma} Y^{2,*}_{i,\gamma} Z^*_{\gamma,\zeta} Y^{3,*}_{b,\zeta} {}^2D^{a,i,b,j} {}^2T_{c,k,a,i} V_{b,c,k,j} \quad (11243)$$

Factorized expression

$$\tau^0_{\gamma,\alpha,w} = \sum_{a \in V} {}^2D^1_{a,w} W^1_{a,\alpha} Y^{1,*}_{a,\gamma} \quad (3r_D r_T r_V N_v) \quad (11244)$$

$$\tau^1_{\gamma,\alpha} = \sum_{a \in V} W^2_{a,\alpha} Y^1_{a,\gamma} \quad (2r_T r_V N_v) \quad (11245)$$

$$\tau^2_{\gamma,\alpha,i} = \sum_{\delta \in A} Y^2_{i,\delta} Z_{\delta,\gamma} \tau^1_{\delta,\alpha} \quad (3r_T^2 r_V N_o) \quad (11246)$$

$$\tau^3_{\gamma,\delta,\alpha,w} = \sum_{i \in O} {}^2D^2_{i,w} Y^{2,*}_{i,\delta} \tau^0_{\delta,\alpha,w} \tau^2_{\gamma,\alpha,i} \quad (4r_D r_T^2 r_V N_o) \quad (11247)$$

$$\tau^4_{\gamma,\alpha} = \sum_{a \in V} W^4_{a,\alpha} Y^3_{a,\gamma} \quad (2r_T r_V N_v) \quad (11248)$$

$$\tau^5_{\gamma,\alpha,a} = \sum_{\beta \in B} X_{\alpha,\beta} W^3_{a,\beta} \tau^4_{\gamma,\beta} \quad (3r_T r_V^2 N_v) \quad (11249)$$

$$\tau^6_{\gamma,\delta,w,a} = \sum_{\alpha \in B} \tau^5_{\gamma,\alpha,a} \tau^3_{\gamma,\delta,\alpha,w} \quad (2r_D r_T^2 r_V N_v) \quad (11250)$$

$$\tau^7_{\gamma,i,a} = \sum_{\delta \in A} \sum_{w \in D} {}^2D^3_{a,w} {}^2D^4_{i,w} Y^4_{i,\delta} \tau^6_{\delta,\gamma,w,a} \quad (4r_D r_T^2 N_o N_v) \quad (11251)$$

$$\tau^8_{\gamma,\delta,i} = \sum_{a \in V} Y^{3,*}_{a,\delta} \tau^7_{\gamma,i,a} \quad (2r_T^2 N_o N_v) \quad (11252)$$

$${}^2R^4_{i,\gamma} \leftarrow \sum_{\delta \in A} \frac{1}{2} Z^*_{\delta,\gamma} \tau^8_{\delta,\gamma,i} \quad (2r_T^2 N_o) \quad (11253)$$

Raw expression

$${}^2R^4_{j,\zeta} \leftarrow - \sum_{\gamma \in A} \sum_{i \in O} \sum_{k \in O} \sum_{a \in V} \sum_{b \in V} \sum_{c \in V} \frac{1}{2} Y^{1,*}_{a,\gamma} Y^{2,*}_{i,\gamma} Z^*_{\gamma,\zeta} Y^{3,*}_{b,\zeta} {}^2D^{a,i,b,j} {}^2T_{c,k,b,j} V_{a,c,k,i} \quad (11254)$$

Factorized expression

$$\tau^0_{\gamma,\alpha,w} = \sum_{a \in V} {}^2D^1_{a,w} W^1_{a,\alpha} Y^{1,*}_{a,\gamma} \quad (3r_D r_T r_V N_v) \quad (11255)$$

$$\tau^1_{\gamma,\alpha} = \sum_{a \in V} W^2_{a,\alpha} Y^3_{a,\gamma} \quad (2r_T r_V N_v) \quad (11256)$$

$$\tau^2_{\gamma,\alpha,i} = \sum_{\delta \in A} Z_{\gamma,\delta} Y^4_{i,\delta} \tau^1_{\delta,\alpha} \quad (3r_T^2 r_V N_o) \quad (11257)$$

$$\tau^3_{\gamma,\delta,\alpha,w} = \sum_{i \in O} {}^2D^2_{i,w} Y^{2,*}_{i,\delta} \tau^0_{\delta,\alpha,w} \tau^2_{\gamma,\alpha,i} \quad (4r_D r_T^2 r_V N_o) \quad (11258)$$

$$\tau^4_{\gamma,\alpha} = \sum_{a \in V} W^4_{a,\alpha} Y^1_{a,\gamma} \quad (2r_T r_V N_v) \quad (11259)$$

$$\tau^5_{\gamma,\alpha,a} = \sum_{\beta \in B} X_{\alpha,\beta} W^3_{a,\beta} \tau^4_{\gamma,\beta} \quad (3r_T r_V^2 N_v) \quad (11260)$$

$$\tau^6_{\gamma,\delta,w,a} = \sum_{\alpha \in B} \tau^5_{\gamma,\alpha,a} \tau^3_{\gamma,\delta,\alpha,w} \quad (2r_D r_T^2 r_V N_v) \quad (11261)$$

$$\tau^7_{\gamma,i,a} = \sum_{\delta \in A} \sum_{w \in D} {}^2D^3_{a,w} {}^2D^4_{i,w} Y^2_{i,\delta} \tau^6_{\delta,\gamma,w,a} \quad (4r_D r_T^2 N_o N_v) \quad (11262)$$

$$\tau^8_{\gamma,\delta,i} = \sum_{a \in V} Y^{3,*}_{a,\delta} \tau^7_{\gamma,i,a} \quad (2r_T^2 N_o N_v) \quad (11263)$$

$${}^2R^4_{i,\gamma} \leftarrow \sum_{\delta \in A} \frac{1}{2} Z^*_{\delta,\gamma} \tau^8_{\delta,\gamma,i} \quad (2r_T^2 N_o) \quad (11264)$$

### E. Contributions from $(H^1 T^1 T^1 T)_c$

Raw expression

$${}^2R^4_{j,\zeta} \leftarrow \sum_{\gamma \in A} \sum_{i \in O} \sum_{k \in O} \sum_{l \in O} \sum_{a \in V} \sum_{b \in V} \sum_{c \in V} {}^1T_{a,k} {}^1T_{b,l} {}^1T_{c,i} Y^{1,*}_{a,\gamma} Y^{2,*}_{i,\gamma} Z^*_{\gamma,\zeta} Y^{3,*}_{b,\zeta} {}^2D^{a,i,b,j}_{k,c,l,j} V_{k,c,l,j} \quad (11265)$$

Factorized expression

$$\tau^0_{\gamma,w,i} = \sum_{a \in V} {}^2D^3_{a,w} {}^1T_{a,i} Y^{3,*}_{a,\gamma} \quad (3r_D r_T N_o N_v) \quad (11266)$$

$$\tau^1_{\gamma,\alpha,w} = \sum_{i \in O} W^3_{i,\alpha} \tau^0_{\gamma,w,i} \quad (2r_D r_T r_V N_o) \quad (11267)$$

$$\tau^2_{\alpha,i} = \sum_{a \in V} {}^1T_{a,i} W^2_{a,\alpha} \quad (2r_V N_o N_v) \quad (11268)$$

$$\tau^3_{\gamma,\alpha,w} = \sum_{i \in O} {}^2D^2_{i,w} Y^{2,*}_{i,\gamma} \tau^2_{\alpha,i} \quad (3r_D r_T r_V N_o) \quad (11269)$$

$$\tau^4_{\gamma,w,i} = \sum_{a \in V} {}^2D^1_{a,w} {}^1T_{a,i} Y^{1,*}_{a,\gamma} \quad (3r_D r_T N_o N_v) \quad (11270)$$

$$\tau^5_{\gamma,\alpha,w} = \sum_{i \in O} W^1_{i,\alpha} \tau^4_{\gamma,w,i} \quad (2r_D r_T r_V N_o) \quad (11271)$$

$$\tau^6_{\gamma,\alpha,w} = \sum_{\beta \in B} X_{\beta,\alpha} \tau^3_{\gamma,\beta,w} \tau^5_{\gamma,\beta,w} \quad (3r_D r_T r_V^2) \quad (11272)$$

$$\tau^7_{\gamma,\alpha,w} = \sum_{\delta \in A} Z^*_{\delta,\gamma} \tau^6_{\delta,\alpha,w} \quad (2r_D r_T^2 r_V) \quad (11273)$$

$$\tau^8_{\gamma,w,i} = \sum_{\alpha \in B} W^4_{i,\alpha} \tau^1_{\gamma,\alpha,w} \tau^7_{\gamma,\alpha,w} \quad (3r_D r_T r_V N_o) \quad (11274)$$

$${}^2R^4_{i,\gamma} \leftarrow \sum_{w \in D} {}^2D^4_{i,w} \tau^8_{\gamma,w,i} \quad (2r_D r_T N_o) \quad (11275)$$

Raw expression

$${}^2R^4_{j,\zeta} \leftarrow \sum_{\gamma \in A} \sum_{i \in O} \sum_{k \in O} \sum_{l \in O} \sum_{a \in V} \sum_{b \in V} \sum_{c \in V} {}^1T_{a,k} {}^1T_{b,l} {}^1T_{c,j} Y^{1,*}_{a,\gamma} Y^{2,*}_{i,\gamma} Z^*_{\gamma,\zeta} Y^{3,*}_{b,\zeta} {}^2D^{a,i,b,j}_{k,c,l,j} V_{k,i,l,c} \quad (11276)$$

Factorized expression

$$\tau^0_{\gamma,w,i} = \sum_{a \in V} {}^2D^3_{a,w} {}^1T_{a,i} Y^{3,*}_{a,\gamma} \quad (3r_D r_T N_o N_v) \quad (11277)$$

$$\tau^1_{\gamma,\alpha,w} = \sum_{i \in O} W^3_{i,\alpha} \tau^0_{\gamma,w,i} \quad (2r_D r_T r_V N_o) \quad (11278)$$

$$\tau^2_{\gamma,\alpha,w} = \sum_{i \in O} {}^2D^2_{i,w} Y^{2,*}_{i,\gamma} \tau^1_{\alpha,i} \quad (3r_D r_T r_V N_o) \quad (11290)$$

$$\tau^2_{\gamma,w,i} = \sum_{a \in V} {}^2D^1_{a,w} {}^1T_{a,i} Y^{1,*}_{a,\gamma} \quad (3r_D r_T N_o N_v) \quad (11279)$$

$$\tau^3_{\gamma,w,i} = \sum_{a \in V} {}^2D^1_{a,w} {}^1T_{a,i} Y^{1,*}_{a,\gamma} \quad (3r_D r_T N_o N_v) \quad (11291)$$

$$\tau^3_{\gamma,\alpha,w} = \sum_{i \in O} W^1_{i,\alpha} \tau^2_{\gamma,w,i} \quad (2r_D r_T r_V N_o) \quad (11280)$$

$$\tau^4_{\gamma,\alpha,w} = \sum_{i \in O} W^3_{i,\alpha} \tau^3_{\gamma,w,i} \quad (2r_D r_T r_V N_o) \quad (11292)$$

$$\tau^4_{\gamma,\alpha,w} = \sum_{i \in O} {}^2D^2_{i,w} W^2_{i,\alpha} Y^{2,*}_{i,\gamma} \quad (3r_D r_T r_V N_o) \quad (11281)$$

$$\tau^5_{\gamma,\alpha,w} = \sum_{\beta \in B} X_{\alpha,\beta} \tau^2_{\gamma,\beta,w} \tau^4_{\gamma,\beta,w} \quad (3r_D r_T r_V^2) \quad (11293)$$

$$\tau^5_{\gamma,\alpha,w} = \sum_{\beta \in B} X_{\beta,\alpha} \tau^3_{\gamma,\beta,w} \tau^4_{\gamma,\beta,w} \quad (3r_D r_T r_V^2) \quad (11282)$$

$$\tau^6_{\gamma,\alpha,w} = \sum_{\delta \in A} Z^*_{\delta,\gamma} \tau^5_{\delta,\alpha,w} \quad (2r_D r_T^2 r_V) \quad (11294)$$

$$\tau^6_{\gamma,\alpha,w} = \sum_{\delta \in A} Z^*_{\delta,\gamma} \tau^5_{\delta,\alpha,w} \quad (2r_D r_T^2 r_V) \quad (11283)$$

$$\tau^7_{\alpha,i} = \sum_{a \in V} {}^1T_{a,i} W^2_{a,\alpha} \quad (2r_V N_o N_v) \quad (11295)$$

$$\tau^7_{\alpha,i} = \sum_{a \in V} {}^1T_{a,i} W^4_{a,\alpha} \quad (2r_V N_o N_v) \quad (11284)$$

$$\tau^8_{\gamma,w,i} = \sum_{\alpha \in B} \tau^7_{\alpha,i} \tau^0_{\gamma,\alpha,w} \tau^6_{\gamma,\alpha,w} \quad (3r_D r_T r_V N_o) \quad (11296)$$

$$\tau^8_{\gamma,w,i} = \sum_{\alpha \in B} \tau^7_{\alpha,i} \tau^1_{\gamma,\alpha,w} \tau^6_{\gamma,\alpha,w} \quad (3r_D r_T r_V N_o) \quad (11285)$$

$${}^2R^4_{i,\gamma} \leftarrow - \sum_{w \in D} {}^2D^4_{i,w} \tau^8_{\gamma,w,i} \quad (2r_D r_T N_o) \quad (11297)$$

$${}^2R^4_{i,\gamma} \leftarrow \sum_{w \in D} {}^2D^4_{i,w} \tau^8_{\gamma,w,i} \quad (2r_D r_T N_o) \quad (11286)$$

Raw expression

$${}^2R^4_{j,\zeta} \leftarrow - \sum_{\gamma \in A} \sum_{i \in O} \sum_{k \in O} \sum_{a \in V} \sum_{b \in V} \sum_{c \in V} \sum_{d \in V} {}^1T_{b,k} {}^1T_{c,i} {}^1T_{d,j} Y^{1,*}_{a,\gamma} Y^{2,*}_{i,\gamma} Z^*_{\gamma,\zeta} Y^{3,*}_{b,\zeta} {}^2D^{a,i,b,j}_{a,c,k,d} V_{a,c,k,d} \quad (11298)$$

Raw expression

$${}^2R^4_{j,\zeta} \leftarrow - \sum_{\gamma \in A} \sum_{i \in O} \sum_{k \in O} \sum_{a \in V} \sum_{b \in V} \sum_{c \in V} \sum_{d \in V} {}^1T_{a,k} {}^1T_{c,i} {}^1T_{d,j} Y^{1,*}_{a,\gamma} Y^{2,*}_{i,\gamma} Z^*_{\gamma,\zeta} Y^{3,*}_{b,\zeta} {}^2D^{a,i,b,j}_{b,d,k,c} V_{b,d,k,c} \quad (11287)$$

Factorized expression

$$\tau^0_{\gamma,w,i} = \sum_{a \in V} {}^2D^3_{a,w} {}^1T_{a,i} Y^{3,*}_{a,\gamma} \quad (3r_D r_T N_o N_v) \quad (11299)$$

Factorized expression

$$\tau^0_{\gamma,\alpha,w} = \sum_{a \in V} {}^2D^3_{a,w} W^1_{a,\alpha} Y^{3,*}_{a,\gamma} \quad (3r_D r_T r_V N_v) \quad (11288)$$

$$\tau^1_{\gamma,\alpha,w} = \sum_{i \in O} W^3_{i,\alpha} \tau^0_{\gamma,w,i} \quad (2r_D r_T r_V N_o) \quad (11300)$$

$$\tau^1_{\alpha,i} = \sum_{a \in V} {}^1T_{a,i} W^4_{a,\alpha} \quad (2r_V N_o N_v) \quad (11289)$$

$$\tau^2_{\alpha,i} = \sum_{a \in V} {}^1T_{a,i} W^2_{a,\alpha} \quad (2r_V N_o N_v) \quad (11301)$$

$$\tau_{\gamma,\alpha,w}^3 = \sum_{i \in O} {}^2D_{i,w}^2 Y_{i,\gamma}^{2,*} \tau_{\alpha,i}^2 \quad (3r_D r_T r_V N_o) \quad (11302)$$

$$\tau_{\gamma,\alpha,w}^4 = \sum_{a \in V} {}^2D_{a,w}^1 W_{a,\alpha}^1 Y_{a,\gamma}^{1,*} \quad (3r_D r_T r_V N_v) \quad (11303)$$

$$\tau_{\gamma,\alpha,w}^5 = \sum_{\beta \in B} X_{\beta,\alpha} \tau_{\gamma,\beta,w}^3 \tau_{\gamma,\beta,w}^4 \quad (3r_D r_T r_V^2) \quad (11304)$$

$$\tau_{\gamma,\alpha,w}^6 = \sum_{\delta \in A} Z_{\delta,\gamma}^* \tau_{\delta,\alpha,w}^5 \quad (2r_D r_T^2 r_V) \quad (11305)$$

$$\tau_{\alpha,i}^7 = \sum_{a \in V} {}^1T_{a,i} W_{a,\alpha}^4 \quad (2r_V N_o N_v) \quad (11306)$$

$$\tau_{\gamma,w,i}^8 = \sum_{\alpha \in B} \tau_{\alpha,i}^7 \tau_{\gamma,\alpha,w}^1 \tau_{\gamma,\alpha,w}^6 \quad (3r_D r_T r_V N_o) \quad (11307)$$

$${}^2R_{i,\gamma}^4 \leftarrow - \sum_{w \in D} {}^2D_{i,w}^4 \tau_{\gamma,w,i}^8 \quad (2r_D r_T N_o) \quad (11308)$$

### F. Contributions from $(H^1 T^2 T)_c$

Raw expression

$${}^2R_{j,\zeta}^4 \leftarrow - \sum_{\gamma \in A} \sum_{i \in O} \sum_{k \in O} \sum_{a \in V} \sum_{b \in V} \sum_{c \in V} \frac{1}{2} {}^1T_{a,k} Y_{a,\gamma}^{1,*} Y_{i,\gamma}^{2,*} Z_{\gamma,\zeta}^* Y_{b,\zeta}^{3,*} f_{k,c} {}^2D_{a,i,b,j} {}^2T_{b,j,c,i} \quad (11309)$$

Factorized expression

$$\tau_{\gamma,\delta,w}^0 = \sum_{a \in V} {}^2D_{a,w}^3 Y_{a,\gamma}^1 Y_{a,\delta}^{3,*} \quad (3r_D r_T^2 N_v) \quad (11310)$$

$$\tau_{\gamma,\delta,w}^1 = \sum_{i \in O} {}^2D_{i,w}^2 Y_{i,\gamma}^4 Y_{i,\delta}^{2,*} \quad (3r_D r_T^2 N_o) \quad (11311)$$

$$\tau_{\gamma,w,i}^2 = \sum_{a \in V} {}^2D_{a,w}^1 {}^1T_{a,i} Y_{a,\gamma}^{1,*} \quad (3r_D r_T N_o N_v) \quad (11312)$$

$$\tau_{\gamma,i}^3 = \sum_{a \in V} Y_{a,\gamma}^3 f_{i,a} \quad (2r_T N_o N_v) \quad (11313)$$

$$\tau_{\gamma,\delta,w}^4 = \sum_{i \in O} \tau_{\gamma,i}^3 \tau_{\delta,w,i}^2 \quad (2r_D r_T^2 N_o) \quad (11314)$$

$$\tau_{\gamma,\delta,w}^5 = \sum_{\epsilon \in A} Z_{\epsilon,\delta}^* \tau_{\gamma,\epsilon,w}^1 \tau_{\gamma,\epsilon,w}^4 \quad (3r_D r_T^3) \quad (11315)$$

$$\tau_{\gamma,\delta,w}^6 = \sum_{\epsilon \in A} Z_{\gamma,\epsilon} \tau_{\epsilon,\delta,w}^5 \quad (2r_D r_T^3) \quad (11316)$$

$${}^2R_{i,\gamma}^4 \leftarrow - \sum_{\delta \in A} \sum_{w \in D} \frac{1}{2} {}^2D_{i,w}^4 Y_{i,\delta}^2 \tau_{\delta,\gamma,w}^0 \tau_{\delta,\gamma,w}^6 \quad (4r_D r_T^2 N_o) \quad (11317)$$

Raw expression

$${}^2R_{j,\zeta}^4 \leftarrow - \sum_{\gamma \in A} \sum_{i \in O} \sum_{k \in O} \sum_{a \in V} \sum_{b \in V} \sum_{c \in V} \frac{1}{2} {}^1T_{a,k} Y_{a,\gamma}^{1,*} Y_{i,\gamma}^{2,*} Z_{\gamma,\zeta}^* Y_{b,\zeta}^{3,*} f_{k,c} {}^2D_{a,i,b,j} {}^2T_{c,i,b,j} \quad (11318)$$

Factorized expression

$$\tau_{\gamma,\delta,w}^0 = \sum_{i \in O} {}^2D_{i,w}^2 Y_{i,\gamma}^2 Y_{i,\delta}^{2,*} \quad (3r_D r_T^2 N_o) \quad (11319)$$

$$\tau_{\gamma,w,i}^1 = \sum_{a \in V} {}^2D_{a,w}^1 {}^1T_{a,i} Y_{a,\gamma}^{1,*} \quad (3r_D r_T N_o N_v) \quad (11320)$$

$$\tau_{\gamma,i}^2 = \sum_{a \in V} Y_{a,\gamma}^1 f_{i,a} \quad (2r_T N_o N_v) \quad (11321)$$

$$\tau_{\gamma,\delta,w}^3 = \sum_{i \in O} \tau_{\gamma,i}^2 \tau_{\delta,w,i}^1 \quad (2r_D r_T^2 N_o) \quad (11322)$$

$$\tau_{\gamma,\delta,w}^4 = \sum_{\epsilon \in A} Z_{\epsilon,\delta}^* \tau_{\gamma,\epsilon,w}^0 \tau_{\gamma,\epsilon,w}^3 \quad (3r_D r_T^3) \quad (11323)$$

$$\tau_{\gamma,\delta,w}^5 = \sum_{\epsilon \in A} Z_{\epsilon,\gamma} \tau_{\epsilon,\delta,w}^4 \quad (2r_D r_T^3) \quad (11324)$$

$$\tau_{\gamma,\delta,w}^6 = \sum_{a \in V} {}^2D_{a,w}^3 Y_{a,\gamma}^3 Y_{a,\delta}^{3,*} \quad (3r_D r_T^2 N_v) \quad (11325)$$

$${}^2R^4_{i,\gamma} \leftarrow - \sum_{\delta \in A} \sum_{w \in D} \frac{1}{2} {}^2D^4_{i,w} Y^4_{i,\delta} \tau^5_{\delta,\gamma,w} \tau^6_{\delta,\gamma,w} \quad (4r_D r_T^2 N_o) \quad (11326)$$

$$\tau^0_{\gamma,w,i} = \sum_{a \in V} {}^2D^3_{a,w} {}^1T_{a,i} Y^{3,*}_{a,\gamma} \quad (3r_D r_T N_o N_v) \quad (11337)$$

Raw expression

$${}^2R^4_{j,\zeta} \leftarrow - \sum_{\gamma \in A} \sum_{i \in O} \sum_{k \in O} \sum_{a \in V} \sum_{b \in V} \sum_{c \in V} \frac{1}{2} {}^1T_{b,k} Y^{1,*}_{a,\gamma} Y^{2,*}_{i,\gamma} Z^*_{\gamma,\zeta} Y^{3,*}_{b,\zeta} f_{k,c} {}^2D^{a,i,b,j} {}^2T_{a,i,c,j} \quad (11327)$$

$$\tau^1_{\gamma,i} = \sum_{a \in V} Y^1_{a,\gamma} f_{i,a} \quad (2r_T N_o N_v) \quad (11338)$$

$$\tau^2_{\gamma,\delta,w} = \sum_{i \in O} \tau^1_{\gamma,i} \tau^0_{\delta,w,i} \quad (2r_D r_T^2 N_o) \quad (11339)$$

Factorized expression

$$\tau^0_{\gamma,\delta,w} = \sum_{a \in V} {}^2D^1_{a,w} Y^1_{a,\gamma} Y^{1,*}_{a,\delta} \quad (3r_D r_T^2 N_v) \quad (11328)$$

$$\tau^3_{\gamma,\delta,w} = \sum_{a \in V} {}^2D^1_{a,w} Y^3_{a,\gamma} Y^{1,*}_{a,\delta} \quad (3r_D r_T^2 N_v) \quad (11340)$$

$$\tau^1_{\gamma,\delta,w} = \sum_{i \in O} {}^2D^2_{i,w} Y^2_{i,\gamma} Y^{2,*}_{i,\delta} \quad (3r_D r_T^2 N_o) \quad (11329)$$

$$\tau^4_{\gamma,\delta,w} = \sum_{i \in O} {}^2D^2_{i,w} Y^4_{i,\gamma} Y^{2,*}_{i,\delta} \quad (3r_D r_T^2 N_o) \quad (11341)$$

$$\tau^2_{\gamma,\delta,w} = \sum_{\epsilon \in A} Z^*_{\epsilon,\delta} \tau^0_{\gamma,\epsilon,w} \tau^1_{\gamma,\epsilon,w} \quad (3r_D r_T^3) \quad (11330)$$

$$\tau^5_{\gamma,\delta,w} = \sum_{\epsilon \in A} Z^*_{\epsilon,\delta} \tau^3_{\gamma,\epsilon,w} \tau^4_{\gamma,\epsilon,w} \quad (3r_D r_T^3) \quad (11342)$$

$$\tau^3_{\gamma,\delta,w} = \sum_{\epsilon \in A} Z_{\epsilon,\gamma} \tau^2_{\epsilon,\delta,w} \quad (2r_D r_T^3) \quad (11331)$$

$$\tau^6_{\gamma,\delta,w} = \sum_{\epsilon \in A} Z_{\gamma,\epsilon} \tau^5_{\epsilon,\delta,w} \quad (2r_D r_T^3) \quad (11343)$$

$$\tau^4_{\gamma,w,i} = \sum_{a \in V} {}^2D^3_{a,w} {}^1T_{a,i} Y^{3,*}_{a,\gamma} \quad (3r_D r_T N_o N_v) \quad (11332)$$

$${}^2R^4_{i,\gamma} \leftarrow - \sum_{\delta \in A} \sum_{w \in D} \frac{1}{2} {}^2D^4_{i,w} Y^2_{i,\delta} \tau^2_{\delta,\gamma,w} \tau^6_{\delta,\gamma,w} \quad (4r_D r_T^2 N_o) \quad (11344)$$

Raw expression

$$\tau^5_{\gamma,i} = \sum_{a \in V} Y^3_{a,\gamma} f_{i,a} \quad (2r_T N_o N_v) \quad (11333)$$

$${}^2R^4_{j,\zeta} \leftarrow - \sum_{\gamma \in A} \sum_{i \in O} \sum_{k \in O} \sum_{a \in V} \sum_{b \in V} \sum_{c \in V} \frac{1}{2} {}^1T_{c,i} Y^{1,*}_{a,\gamma} Y^{2,*}_{i,\gamma} Z^*_{\gamma,\zeta} Y^{3,*}_{b,\zeta} f_{k,c} {}^2D^{a,i,b,j} {}^2T_{a,k,b,j} \quad (11345)$$

$$\tau^6_{\gamma,\delta,w} = \sum_{i \in O} \tau^5_{\gamma,i} \tau^4_{\delta,w,i} \quad (2r_D r_T^2 N_o) \quad (11334)$$

Factorized expression

$${}^2R^4_{i,\gamma} \leftarrow - \sum_{\delta \in A} \sum_{w \in D} \frac{1}{2} {}^2D^4_{i,w} Y^4_{i,\delta} \tau^3_{\delta,\gamma,w} \tau^6_{\delta,\gamma,w} \quad (4r_D r_T^2 N_o) \quad (11335)$$

$$\tau^0_{\gamma,\delta,w} = \sum_{a \in V} {}^2D^1_{a,w} Y^1_{a,\gamma} Y^{1,*}_{a,\delta} \quad (3r_D r_T^2 N_v) \quad (11346)$$

Raw expression

$${}^2R^4_{j,\zeta} \leftarrow - \sum_{\gamma \in A} \sum_{i \in O} \sum_{k \in O} \sum_{a \in V} \sum_{b \in V} \sum_{c \in V} \frac{1}{2} {}^1T_{b,k} Y^{1,*}_{a,\gamma} Y^{2,*}_{i,\gamma} Z^*_{\gamma,\zeta} Y^{3,*}_{b,\zeta} f_{k,c} {}^2D^{a,i,b,j} {}^2T_{c,j,a,i} \quad (11336)$$

$$\tau^1_{i,j} = \sum_{a \in V} {}^1T_{a,i} f_{j,a} \quad (2N_o^2 N_v) \quad (11347)$$

$$\tau^2_{\gamma,i} = \sum_{j \in O} Y^2_{j,\gamma} \tau^1_{i,j} \quad (2r_T N_o^2) \quad (11348)$$

Factorized expression

$$\tau^3_{\gamma,\delta,w} = \sum_{i \in O} {}^2D^2_{i,w} Y^{2,*}_{i,\delta} \tau^2_{\gamma,i} \quad (3r_D r_T^2 N_o) \quad (11349)$$

$$\tau^4_{\gamma,\delta,w} = \sum_{\epsilon \in A} Z^*_{\epsilon,\delta} \tau^0_{\gamma,\epsilon,w} \tau^3_{\gamma,\epsilon,w} \quad (3r_D r_T^3) \quad (11350)$$

$$\tau^5_{\gamma,\delta,w} = \sum_{\epsilon \in A} Z_{\epsilon,\gamma} \tau^4_{\epsilon,\delta,w} \quad (2r_D r_T^3) \quad (11351)$$

$$\tau^6_{\gamma,\delta,w} = \sum_{a \in V} {}^2D^3_{a,w} Y^3_{a,\gamma} Y^{3,*}_{a,\delta} \quad (3r_D r_T^2 N_v) \quad (11352)$$

$${}^2R^4_{i,\gamma} \leftarrow - \sum_{\delta \in A} \sum_{w \in D} \frac{1}{2} {}^2D^4_{i,w} Y^4_{i,\delta} \tau^5_{\delta,\gamma,w} \tau^6_{\delta,\gamma,w} \quad (4r_D r_T^2 N_o) \quad (11353)$$

Raw expression

$${}^2R^4_{j,\zeta} \leftarrow - \sum_{\gamma \in A} \sum_{i \in O} \sum_{k \in O} \sum_{a \in V} \sum_{b \in V} \sum_{c \in V} \frac{1}{2} {}^1T_{c,i} Y^{1,*}_{a,\gamma} Y^{2,*}_{i,\gamma} Z^*_{\gamma,\zeta} Y^{3,*}_{b,\zeta} f_{k,c} {}^2D^{a,i,b,j} {}^2T_{b,j,a,k} \quad (11354)$$

Factorized expression

$$\tau^0_{\gamma,\delta,w} = \sum_{a \in V} {}^2D^1_{a,w} Y^3_{a,\gamma} Y^{1,*}_{a,\delta} \quad (3r_D r_T^2 N_v) \quad (11355)$$

$$\tau^1_{i,j} = \sum_{a \in V} {}^1T_{a,i} f_{j,a} \quad (2N_o^2 N_v) \quad (11356)$$

$$\tau^2_{\gamma,i} = \sum_{j \in O} Y^4_{j,\gamma} \tau^1_{i,j} \quad (2r_T N_o^2) \quad (11357)$$

$$\tau^3_{\gamma,\delta,w} = \sum_{i \in O} {}^2D^2_{i,w} Y^{2,*}_{i,\delta} \tau^2_{\gamma,i} \quad (3r_D r_T^2 N_o) \quad (11358)$$

$$\tau^4_{\gamma,\delta,w} = \sum_{\epsilon \in A} Z^*_{\epsilon,\delta} \tau^0_{\gamma,\epsilon,w} \tau^3_{\gamma,\epsilon,w} \quad (3r_D r_T^3) \quad (11359)$$

$$\tau^5_{\gamma,\delta,w} = \sum_{\epsilon \in A} Z_{\gamma,\epsilon} \tau^4_{\epsilon,\delta,w} \quad (2r_D r_T^3) \quad (11360)$$

$$\tau^6_{\gamma,\delta,w} = \sum_{a \in V} {}^2D^3_{a,w} Y^1_{a,\gamma} Y^{3,*}_{a,\delta} \quad (3r_D r_T^2 N_v) \quad (11361)$$

$${}^2R^4_{i,\gamma} \leftarrow - \sum_{\delta \in A} \sum_{w \in D} \frac{1}{2} {}^2D^4_{i,w} Y^2_{i,\delta} \tau^5_{\delta,\gamma,w} \tau^6_{\delta,\gamma,w} \quad (4r_D r_T^2 N_o) \quad (11362)$$

Raw expression

$${}^2R^4_{j,\zeta} \leftarrow - \sum_{\gamma \in A} \sum_{i \in O} \sum_{k \in O} \sum_{a \in V} \sum_{b \in V} \sum_{c \in V} \frac{1}{2} {}^1T_{c,j} Y^{1,*}_{a,\gamma} Y^{2,*}_{i,\gamma} Z^*_{\gamma,\zeta} Y^{3,*}_{b,\zeta} f_{k,c} {}^2D^{a,i,b,j} {}^2T_{a,i,b,k} \quad (11363)$$

Factorized expression

$$\tau^0_{\gamma,\delta,w} = \sum_{a \in V} {}^2D^3_{a,w} Y^3_{a,\gamma} Y^{3,*}_{a,\delta} \quad (3r_D r_T^2 N_v) \quad (11364)$$

$$\tau^1_{\gamma,\delta,w} = \sum_{a \in V} {}^2D^1_{a,w} Y^1_{a,\gamma} Y^{1,*}_{a,\delta} \quad (3r_D r_T^2 N_v) \quad (11365)$$

$$\tau^2_{\gamma,\delta,w} = \sum_{i \in O} {}^2D^2_{i,w} Y^2_{i,\gamma} Y^{2,*}_{i,\delta} \quad (3r_D r_T^2 N_o) \quad (11366)$$

$$\tau^3_{\gamma,\delta,w} = \sum_{\epsilon \in A} Z^*_{\epsilon,\delta} \tau^1_{\gamma,\epsilon,w} \tau^2_{\gamma,\epsilon,w} \quad (3r_D r_T^3) \quad (11367)$$

$$\tau^4_{\gamma,\delta,w} = \sum_{\epsilon \in A} Z_{\epsilon,\gamma} \tau^3_{\epsilon,\delta,w} \quad (2r_D r_T^3) \quad (11368)$$

$$\tau^5_{i,j} = \sum_{a \in V} {}^1T_{a,i} f_{j,a} \quad (2N_o^2 N_v) \quad (11369)$$

$$\tau^6_{\gamma,i} = \sum_{j \in O} Y^4_{j,\gamma} \tau^5_{i,j} \quad (2r_T N_o^2) \quad (11370)$$

$${}^2R^4_{i,\gamma} \leftarrow - \sum_{\delta \in A} \sum_{w \in D} \frac{1}{2} {}^2D^4_{i,w} \tau^6_{\delta,i} \tau^0_{\delta,\gamma,w} \tau^4_{\delta,\gamma,w} \quad (4r_D r_T^2 N_o) \quad (11371)$$

Raw expression

$${}^2R^4_{j,\zeta} \leftarrow - \sum_{\gamma \in A} \sum_{i \in O} \sum_{k \in O} \sum_{a \in V} \sum_{b \in V} \sum_{c \in V} \frac{1}{2} {}^1T_{c,j} Y^{1,*}_{a,\gamma} Y^{2,*}_{i,\gamma} Z^*_{\gamma,\zeta} Y^{3,*}_{b,\zeta} f_{k,c} {}^2D^{a,i,b,j} {}^2T_{b,k,a,i} \quad (11372)$$

Factorized expression



$$\tau^0_{\gamma,\delta,w} = \sum_{a \in V} {}^2D^3_{a,w} Y^1_{a,\gamma} Y^{3,*}_{a,\delta} \quad (3r_D r_T^2 N_v) \quad (11373)$$

$$\tau^3_{\gamma,\alpha,w} = \sum_{a \in V} {}^2D^1_{a,w} W^1_{a,\alpha} Y^{1,*}_{a,\gamma} \quad (3r_D r_T r_V N_v) \quad (11385)$$

$$\tau^1_{\gamma,\delta,w} = \sum_{a \in V} {}^2D^1_{a,w} Y^3_{a,\gamma} Y^{1,*}_{a,\delta} \quad (3r_D r_T^2 N_v) \quad (11374)$$

$$\tau^4_{\gamma,\alpha} = \sum_{a \in V} W^4_{a,\alpha} Y^3_{a,\gamma} \quad (2r_T r_V N_v) \quad (11386)$$

$$\tau^2_{\gamma,\delta,w} = \sum_{i \in O} {}^2D^2_{i,w} Y^4_{i,\gamma} Y^{2,*}_{i,\delta} \quad (3r_D r_T^2 N_o) \quad (11375)$$

$$\tau^5_{\gamma,\alpha} = \sum_{i \in O} W^3_{i,\alpha} Y^4_{i,\gamma} \quad (2r_T r_V N_o) \quad (11387)$$

$$\tau^3_{\gamma,\delta,w} = \sum_{\epsilon \in A} Z^*_{\epsilon,\delta} \tau^1_{\gamma,\epsilon,w} \tau^2_{\gamma,\epsilon,w} \quad (3r_D r_T^3) \quad (11376)$$

$$\tau^6_{\gamma,\alpha} = \sum_{\beta \in B} X_{\alpha,\beta} \tau^4_{\gamma,\beta} \tau^5_{\gamma,\beta} \quad (3r_T r_V^2) \quad (11388)$$

$$\tau^4_{\gamma,\delta,w} = \sum_{\epsilon \in A} Z_{\gamma,\epsilon} \tau^3_{\epsilon,\delta,w} \quad (2r_D r_T^3) \quad (11377)$$

$$\tau^7_{\gamma,\alpha} = \sum_{\delta \in A} Z_{\gamma,\delta} \tau^6_{\delta,\alpha} \quad (2r_T^2 r_V) \quad (11389)$$

$$\tau^5_{i,j} = \sum_{a \in V} {}^1T_{a,i} f_{j,a} \quad (2N_o^2 N_v) \quad (11378)$$

$$\tau^8_{\gamma,\delta,w} = \sum_{\alpha \in B} \tau^7_{\gamma,\alpha} \tau^2_{\delta,\alpha,w} \tau^3_{\delta,\alpha,w} \quad (3r_D r_T^2 r_V) \quad (11390)$$

$$\tau^6_{\gamma,i} = \sum_{j \in O} Y^2_{j,\gamma} \tau^5_{i,j} \quad (2r_T N_o^2) \quad (11379)$$

$$\tau^9_{\gamma,\delta,w} = \sum_{\epsilon \in A} Z^*_{\epsilon,\delta} \tau^8_{\gamma,\epsilon,w} \quad (2r_D r_T^3) \quad (11391)$$

$${}^2R^4_{i,\gamma} \leftarrow - \sum_{\delta \in A} \sum_{w \in D} \frac{1}{2} {}^2D^4_{i,w} \tau^6_{\delta,i} \tau^0_{\delta,\gamma,w} \tau^4_{\delta,\gamma,w} \quad (4r_D r_T^2 N_o) {}^2R^4_{i,\gamma} \leftarrow \sum_{\delta \in A} \sum_{w \in D} {}^2D^4_{i,w} Y^2_{i,\delta} \tau^0_{\delta,\gamma,w} \tau^9_{\delta,\gamma,w} \quad (4r_D r_T^2 N_o) \quad (11380) \quad (11392)$$

Raw expression

$${}^2R^4_{j,\zeta} \leftarrow \sum_{\gamma \in A} \sum_{i \in O} \sum_{k \in O} \sum_{a \in V} \sum_{b \in V} \sum_{c \in V} \sum_{d \in V} {}^1T_{c,i} Y^{1,*}_{a,\gamma} Y^{2,*}_{i,\gamma} Z^*_{\gamma,\zeta} Y^{3,*}_{b,\zeta} {}^2D^{a,i,b,j} {}^2T_{b,j,d,k} V_{a,c,k,d} \quad (11381)$$

Raw expression

$${}^2R^4_{j,\zeta} \leftarrow \sum_{\gamma \in A} \sum_{i \in O} \sum_{k \in O} \sum_{a \in V} \sum_{b \in V} \sum_{c \in V} \sum_{d \in V} {}^1T_{c,i} Y^{1,*}_{a,\gamma} Y^{2,*}_{i,\gamma} Z^*_{\gamma,\zeta} Y^{3,*}_{b,\zeta} {}^2D^{a,i,b,j} {}^2T_{d,k,b,j} V_{a,c,k,d} \quad (11393)$$

Factorized expression

$$\tau^0_{\gamma,\delta,w} = \sum_{a \in V} {}^2D^3_{a,w} Y^1_{a,\gamma} Y^{3,*}_{a,\delta} \quad (3r_D r_T^2 N_v) \quad (11382)$$

$$\tau^0_{\gamma,\delta,w} = \sum_{a \in V} {}^2D^3_{a,w} Y^3_{a,\gamma} Y^{3,*}_{a,\delta} \quad (3r_D r_T^2 N_v) \quad (11394)$$

$$\tau^1_{\alpha,i} = \sum_{a \in V} {}^1T_{a,i} W^2_{a,\alpha} \quad (2r_V N_o N_v) \quad (11383)$$

$$\tau^1_{\alpha,i} = \sum_{a \in V} {}^1T_{a,i} W^2_{a,\alpha} \quad (2r_V N_o N_v) \quad (11395)$$

$$\tau^2_{\gamma,\alpha,w} = \sum_{i \in O} {}^2D^2_{i,w} Y^{2,*}_{i,\gamma} \tau^1_{\alpha,i} \quad (3r_D r_T r_V N_o) \quad (11384)$$

$$\tau^2_{\gamma,\alpha,w} = \sum_{i \in O} {}^2D^2_{i,w} Y^{2,*}_{i,\gamma} \tau^1_{\alpha,i} \quad (3r_D r_T r_V N_o) \quad (11396)$$

$$\tau^3_{\gamma,\alpha,w} = \sum_{a \in V} {}^2D^1_{a,w} W^1_{a,\alpha} Y^{1,*}_{a,\gamma} \quad (3r_D r_T r_V N_v) \quad (11397)$$

$$\tau^4_{\gamma,\alpha} = \sum_{a \in V} W^4_{a,\alpha} Y^1_{a,\gamma} \quad (2r_T r_V N_v) \quad (11398)$$

$$\tau^5_{\gamma,\alpha} = \sum_{i \in O} W^3_{i,\alpha} Y^2_{i,\gamma} \quad (2r_T r_V N_o) \quad (11399)$$

$$\tau^6_{\gamma,\alpha} = \sum_{\beta \in B} X_{\alpha,\beta} \tau^4_{\gamma,\beta} \tau^5_{\gamma,\beta} \quad (3r_T r_V^2) \quad (11400)$$

$$\tau^7_{\gamma,\alpha} = \sum_{\delta \in A} Z_{\delta,\gamma} \tau^6_{\delta,\alpha} \quad (2r_T^2 r_V) \quad (11401)$$

$$\tau^8_{\gamma,\delta,w} = \sum_{\alpha \in B} \tau^7_{\gamma,\alpha} \tau^2_{\delta,\alpha,w} \tau^3_{\delta,\alpha,w} \quad (3r_D r_T^2 r_V) \quad (11402)$$

$$\tau^9_{\gamma,\delta,w} = \sum_{\epsilon \in A} Z^*_{\epsilon,\delta} \tau^8_{\gamma,\epsilon,w} \quad (2r_D r_T^3) \quad (11403)$$

$${}^2R^4_{i,\gamma} \leftarrow \sum_{\delta \in A} \sum_{w \in D} {}^2D^4_{i,w} Y^4_{i,\delta} \tau^0_{\delta,\gamma,w} \tau^9_{\delta,\gamma,w} \quad (4r_D r_T^2 N_o) \quad (11404)$$

Raw expression

$${}^2R^4_{j,\zeta} \leftarrow \sum_{\gamma \in A} \sum_{i \in O} \sum_{k \in O} \sum_{a \in V} \sum_{b \in V} \sum_{c \in V} \sum_{d \in V} {}^1T_{c,j} Y^{1,*}_{a,\gamma} Y^{2,*}_{i,\gamma} Z^*_{\gamma,\zeta} Y^{3,*}_{b,\zeta} {}^2D^{a,i,b,j} {}^2T_{a,i,d,k} V_{b,c,k,d} \quad (11405)$$

Factorized expression

$$\tau^0_{\gamma,\alpha,w} = \sum_{a \in V} {}^2D^3_{a,w} W^1_{a,\alpha} Y^{3,*}_{a,\gamma} \quad (3r_D r_T r_V N_v) \quad (11406)$$

$$\tau^1_{\gamma,\alpha} = \sum_{a \in V} W^4_{a,\alpha} Y^3_{a,\gamma} \quad (2r_T r_V N_v) \quad (11407)$$

$$\tau^2_{\gamma,\alpha} = \sum_{i \in O} W^3_{i,\alpha} Y^4_{i,\gamma} \quad (2r_T r_V N_o) \quad (11408)$$

$$\tau^3_{\gamma,\alpha} = \sum_{\beta \in B} X_{\alpha,\beta} \tau^1_{\gamma,\beta} \tau^2_{\gamma,\beta} \quad (3r_T r_V^2) \quad (11409)$$

$$\tau^4_{\gamma,\alpha} = \sum_{\delta \in A} Z_{\gamma,\delta} \tau^3_{\delta,\alpha} \quad (2r_T^2 r_V) \quad (11410)$$

$$\tau^5_{\gamma,\delta,w} = \sum_{a \in V} {}^2D^1_{a,w} Y^1_{a,\gamma} Y^{1,*}_{a,\delta} \quad (3r_D r_T^2 N_v) \quad (11411)$$

$$\tau^6_{\gamma,\delta,w} = \sum_{i \in O} {}^2D^2_{i,w} Y^2_{i,\gamma} Y^{2,*}_{i,\delta} \quad (3r_D r_T^2 N_o) \quad (11412)$$

$$\tau^7_{\gamma,\delta,w} = \sum_{\epsilon \in A} Z^*_{\epsilon,\delta} \tau^5_{\gamma,\epsilon,w} \tau^6_{\gamma,\epsilon,w} \quad (3r_D r_T^3) \quad (11413)$$

$$\tau^8_{\gamma,\alpha,w} = \sum_{\delta \in A} \tau^4_{\delta,\alpha} \tau^7_{\delta,\gamma,w} \quad (2r_D r_T^2 r_V) \quad (11414)$$

$$\tau^9_{\alpha,i} = \sum_{a \in V} {}^1T_{a,i} W^2_{a,\alpha} \quad (2r_V N_o N_v) \quad (11415)$$

$$\tau^{10}_{\gamma,w,i} = \sum_{\alpha \in B} \tau^9_{\alpha,i} \tau^0_{\gamma,\alpha,w} \tau^8_{\gamma,\alpha,w} \quad (3r_D r_T r_V N_o) \quad (11416)$$

$${}^2R^4_{i,\gamma} \leftarrow \sum_{w \in D} {}^2D^4_{i,w} \tau^{10}_{\gamma,w,i} \quad (2r_D r_T N_o) \quad (11417)$$

Raw expression

$${}^2R^4_{j,\zeta} \leftarrow \sum_{\gamma \in A} \sum_{i \in O} \sum_{k \in O} \sum_{a \in V} \sum_{b \in V} \sum_{c \in V} \sum_{d \in V} {}^1T_{c,j} Y^{1,*}_{a,\gamma} Y^{2,*}_{i,\gamma} Z^*_{\gamma,\zeta} Y^{3,*}_{b,\zeta} {}^2D^{a,i,b,j} {}^2T_{d,k,a,i} V_{b,c,k,d} \quad (11418)$$

Factorized expression

$$\tau^0_{\gamma,\alpha,w} = \sum_{a \in V} {}^2D^3_{a,w} W^1_{a,\alpha} Y^{3,*}_{a,\gamma} \quad (3r_D r_T r_V N_v) \quad (11419)$$

$$\tau^1_{\gamma,\delta,w} = \sum_{a \in V} {}^2D^1_{a,w} Y^3_{a,\gamma} Y^{1,*}_{a,\delta} \quad (3r_D r_T^2 N_v) \quad (11420)$$

$$\tau_{\gamma,\delta,w}^2 = \sum_{i \in O} {}^2D_{i,w}^2 Y_{i,\gamma}^4 Y_{i,\delta}^{2,*} \quad (3r_D r_T^2 N_o) \quad (11421)$$

$$\tau_{\alpha,i}^2 = \sum_{a \in V} {}^1T_{a,i} W_{a,\alpha}^4 \quad (2r_V N_o N_v) \quad (11434)$$

$$\tau_{\gamma,\delta,w}^3 = \sum_{\epsilon \in A} Z_{\epsilon,\delta}^* \tau_{\gamma,\epsilon,w}^1 \tau_{\gamma,\epsilon,w}^2 \quad (3r_D r_T^3) \quad (11422)$$

$$\tau_{\alpha}^3 = \sum_{i \in O} W_{i,\alpha}^3 \tau_{\alpha,i}^2 \quad (2r_V N_o) \quad (11435)$$

$$\tau_{\gamma,\alpha}^4 = \sum_{a \in V} W_{a,\alpha}^4 Y_{a,\gamma}^1 \quad (2r_T r_V N_v) \quad (11423)$$

$$\tau_{\alpha}^4 = \sum_{\beta \in B} \tau_{\beta}^3 X_{\alpha,\beta} \quad (2r_V^2) \quad (11436)$$

$$\tau_{\gamma,\alpha}^5 = \sum_{i \in O} W_{i,\alpha}^3 Y_{i,\gamma}^2 \quad (2r_T r_V N_o) \quad (11424)$$

$$\tau_{a,b}^5 = \sum_{\alpha \in B} \tau_{\alpha}^4 W_{a,\alpha}^1 W_{b,\alpha}^2 \quad (3r_V N_v^2) \quad (11437)$$

$$\tau_{\gamma,\alpha}^6 = \sum_{\beta \in B} X_{\alpha,\beta} \tau_{\gamma,\beta}^4 \tau_{\gamma,\beta}^5 \quad (3r_T r_V^2) \quad (11425)$$

$$\tau_{\gamma,a}^6 = \sum_{b \in V} Y_{b,\gamma}^3 \tau_{a,b}^5 \quad (2r_T N_v^2) \quad (11438)$$

$$\tau_{\gamma,\alpha}^7 = \sum_{\delta \in A} Z_{\delta,\gamma} \tau_{\delta,\alpha}^6 \quad (2r_T^2 r_V) \quad (11426)$$

$$\tau_{\gamma,\delta,w}^7 = \sum_{a \in V} {}^2D_{a,w}^1 Y_{a,\delta}^{1,*} \tau_{\gamma,a}^6 \quad (3r_D r_T^2 N_v) \quad (11439)$$

$$\tau_{\gamma,\alpha,w}^8 = \sum_{\delta \in A} \tau_{\delta,\alpha}^7 \tau_{\delta,\gamma,w}^3 \quad (2r_D r_T^2 r_V) \quad (11427)$$

$$\tau_{\gamma,\delta,w}^8 = \sum_{\epsilon \in A} Z_{\epsilon,\delta}^* \tau_{\gamma,\epsilon,w}^1 \tau_{\gamma,\epsilon,w}^7 \quad (3r_D r_T^3) \quad (11440)$$

$$\tau_{\alpha,i}^9 = \sum_{a \in V} {}^1T_{a,i} W_{a,\alpha}^2 \quad (2r_V N_o N_v) \quad (11428)$$

$$\tau_{\gamma,\delta,w}^9 = \sum_{\epsilon \in A} Z_{\gamma,\epsilon} \tau_{\epsilon,\delta,w}^8 \quad (2r_D r_T^3) \quad (11441)$$

$$\tau_{\gamma,w,i}^{10} = \sum_{\alpha \in B} \tau_{\alpha,i}^9 \tau_{\gamma,\alpha,w}^0 \tau_{\gamma,\alpha,w}^8 \quad (3r_D r_T r_V N_o) \quad (11429)$$

$${}^2R_{i,\gamma}^4 \leftarrow \sum_{\delta \in A} \sum_{w \in D} {}^2D_{i,w}^4 Y_{i,\delta}^2 \tau_{\delta,\gamma,w}^0 \tau_{\delta,\gamma,w}^9 \quad (4r_D r_T^2 N_o) \quad (11442)$$

$${}^2R_{i,\gamma}^4 \leftarrow \sum_{w \in D} {}^2D_{i,w}^4 \tau_{\gamma,w,i}^{10} \quad (2r_D r_T N_o) \quad (11430)$$

Raw expression

$${}^2R_{j,\zeta}^4 \leftarrow \sum_{\gamma \in A} \sum_{i \in O} \sum_{k \in O} \sum_{a \in V} \sum_{b \in V} \sum_{c \in V} \sum_{d \in V} {}^1T_{c,k} Y_{a,\gamma}^{1,*} Y_{i,\gamma}^{2,*} Z_{\gamma,\zeta}^* Y_{b,\zeta}^{3,*} {}^2D_{a,i,b,j} {}^2T_{b,j,d,i} V_{a,d,k,c} \quad (11443)$$

Raw expression

$${}^2R_{j,\zeta}^4 \leftarrow \sum_{\gamma \in A} \sum_{i \in O} \sum_{k \in O} \sum_{a \in V} \sum_{b \in V} \sum_{c \in V} \sum_{d \in V} {}^1T_{c,k} Y_{a,\gamma}^{1,*} Y_{i,\gamma}^{2,*} Z_{\gamma,\zeta}^* Y_{b,\zeta}^{3,*} {}^2D_{a,i,b,j} {}^2T_{a,i,d,j} V_{b,d,k,c} \quad (11431)$$

Factorized expression

$$\tau_{\gamma,\delta,w}^0 = \sum_{a \in V} {}^2D_{a,w}^3 Y_{a,\gamma}^3 Y_{a,\delta}^{3,*} \quad (3r_D r_T^2 N_v) \quad (11444)$$

Factorized expression

$$\tau_{\gamma,\delta,w}^0 = \sum_{a \in V} {}^2D_{a,w}^3 Y_{a,\gamma}^1 Y_{a,\delta}^{3,*} \quad (3r_D r_T^2 N_v) \quad (11432)$$

$$\tau_{\gamma,\delta,w}^1 = \sum_{i \in O} {}^2D_{i,w}^2 Y_{i,\gamma}^2 Y_{i,\delta}^{2,*} \quad (3r_D r_T^2 N_o) \quad (11445)$$

$$\tau_{\gamma,\delta,w}^1 = \sum_{i \in O} {}^2D_{i,w}^2 Y_{i,\gamma}^4 Y_{i,\delta}^{2,*} \quad (3r_D r_T^2 N_o) \quad (11433)$$

$$\tau_{\alpha,i}^2 = \sum_{a \in V} {}^1T_{a,i} W_{a,\alpha}^4 \quad (2r_V N_o N_v) \quad (11446)$$

$$\tau^3_{\alpha} = \sum_{i \in O} W^3_{i,\alpha} \tau^2_{\alpha,i} \quad (2r_V N_o) \quad (11447)$$

$$\tau^4_{\gamma,a} = \sum_{b \in V} Y^3_{b,\gamma} \tau^3_{a,b} \quad (2r_T N_v^2) \quad (11460)$$

$$\tau^4_{\alpha} = \sum_{\beta \in B} \tau^3_{\beta} X_{\alpha,\beta} \quad (2r_V^2) \quad (11448)$$

$$\tau^5_{\gamma,\delta,w} = \sum_{a \in V} {}^2D^3_{a,w} Y^{3,*}_{a,\delta} \tau^4_{\gamma,a} \quad (3r_D r_T^2 N_v) \quad (11461)$$

$$\tau^5_{a,b} = \sum_{\alpha \in B} \tau^4_{\alpha} W^1_{a,\alpha} W^2_{b,\alpha} \quad (3r_V N_v^2) \quad (11449)$$

$$\tau^6_{\gamma,\delta,w} = \sum_{a \in V} {}^2D^1_{a,w} Y^1_{a,\gamma} Y^{1,*}_{a,\delta} \quad (3r_D r_T^2 N_v) \quad (11462)$$

$$\tau^6_{\gamma,a} = \sum_{b \in V} Y^1_{b,\gamma} \tau^5_{a,b} \quad (2r_T N_v^2) \quad (11450)$$

$$\tau^7_{\gamma,\delta,w} = \sum_{i \in O} {}^2D^2_{i,w} Y^2_{i,\gamma} Y^{2,*}_{i,\delta} \quad (3r_D r_T^2 N_o) \quad (11463)$$

$$\tau^7_{\gamma,\delta,w} = \sum_{a \in V} {}^2D^1_{a,w} Y^{1,*}_{a,\delta} \tau^6_{\gamma,a} \quad (3r_D r_T^2 N_v) \quad (11451)$$

$$\tau^8_{\gamma,\delta,w} = \sum_{\epsilon \in A} Z^*_{\epsilon,\delta} \tau^6_{\gamma,\epsilon,w} \tau^7_{\gamma,\epsilon,w} \quad (3r_D r_T^3) \quad (11464)$$

$$\tau^8_{\gamma,\delta,w} = \sum_{\epsilon \in A} Z^*_{\epsilon,\delta} \tau^1_{\gamma,\epsilon,w} \tau^7_{\gamma,\epsilon,w} \quad (3r_D r_T^3) \quad (11452)$$

$$\tau^9_{\gamma,\delta,w} = \sum_{\epsilon \in A} Z_{\epsilon,\gamma} \tau^8_{\epsilon,\delta,w} \quad (2r_D r_T^3) \quad (11465)$$

$$\tau^9_{\gamma,\delta,w} = \sum_{\epsilon \in A} Z_{\epsilon,\gamma} \tau^8_{\epsilon,\delta,w} \quad (2r_D r_T^3) \quad (11453)$$

$${}^2R^4_{i,\gamma} \leftarrow \sum_{\delta \in A} \sum_{w \in D} {}^2D^4_{i,w} Y^4_{i,\delta} \tau^5_{\delta,\gamma,w} \tau^9_{\delta,\gamma,w} \quad (4r_D r_T^2 N_o) \quad (11466)$$

$${}^2R^4_{i,\gamma} \leftarrow \sum_{\delta \in A} \sum_{w \in D} {}^2D^4_{i,w} Y^4_{i,\delta} \tau^0_{\delta,\gamma,w} \tau^9_{\delta,\gamma,w} \quad (4r_D r_T^2 N_o) \quad (11454)$$

Raw expression

$${}^2R^4_{j,\zeta} \leftarrow \sum_{\gamma \in A} \sum_{i \in O} \sum_{k \in O} \sum_{a \in V} \sum_{b \in V} \sum_{c \in V} \sum_{d \in V} {}^1T_{c,k} Y^{1,*}_{a,\gamma} Y^{2,*}_{i,\gamma} Z^*_{\gamma,\zeta} Y^{3,*}_{b,\zeta} {}^2D^{a,i,b,j} {}^2T_{d,j,a,i} V_{b,d,k,c} \quad (11467)$$

Raw expression

$${}^2R^4_{j,\zeta} \leftarrow \sum_{\gamma \in A} \sum_{i \in O} \sum_{k \in O} \sum_{a \in V} \sum_{b \in V} \sum_{c \in V} \sum_{d \in V} {}^1T_{c,k} Y^{1,*}_{a,\gamma} Y^{2,*}_{i,\gamma} Z^*_{\gamma,\zeta} Y^{3,*}_{b,\zeta} {}^2D^{a,i,b,j} {}^2T_{d,i,b,j} V_{a,d,k,c} \quad (11455)$$

Factorized expression

$$\tau^0_{\alpha,i} = \sum_{a \in V} {}^1T_{a,i} W^4_{a,\alpha} \quad (2r_V N_o N_v) \quad (11468)$$

Factorized expression

$$\tau^0_{\alpha,i} = \sum_{a \in V} {}^1T_{a,i} W^4_{a,\alpha} \quad (2r_V N_o N_v) \quad (11456)$$

$$\tau^1_{\alpha} = \sum_{i \in O} W^3_{i,\alpha} \tau^0_{\alpha,i} \quad (2r_V N_o) \quad (11469)$$

$$\tau^1_{\alpha} = \sum_{i \in O} W^3_{i,\alpha} \tau^0_{\alpha,i} \quad (2r_V N_o) \quad (11457)$$

$$\tau^2_{\alpha} = \sum_{\beta \in B} \tau^1_{\beta} X_{\alpha,\beta} \quad (2r_V^2) \quad (11470)$$

$$\tau^2_{\alpha} = \sum_{\beta \in B} \tau^1_{\beta} X_{\alpha,\beta} \quad (2r_V^2) \quad (11458)$$

$$\tau^3_{a,b} = \sum_{\alpha \in B} \tau^2_{\alpha} W^1_{a,\alpha} W^2_{b,\alpha} \quad (3r_V N_v^2) \quad (11471)$$

$$\tau^3_{a,b} = \sum_{\alpha \in B} \tau^2_{\alpha} W^1_{a,\alpha} W^2_{b,\alpha} \quad (3r_V N_v^2) \quad (11459)$$

$$\tau^4_{\gamma,a} = \sum_{b \in V} Y^1_{b,\gamma} \tau^3_{a,b} \quad (2r_T N_v^2) \quad (11472)$$

$$\tau^5_{\gamma,\delta,w} = \sum_{a \in V} {}^2D^3_{a,w} Y^{3,*}_{a,\delta} \tau^4_{\gamma,a} \quad (3r_D r_T^2 N_v) \quad (11473)$$

$$\tau^6_{\gamma,\delta,w} = \sum_{a \in V} {}^2D^1_{a,w} Y^3_{a,\gamma} Y^{1,*}_{a,\delta} \quad (3r_D r_T^2 N_v) \quad (11474)$$

$$\tau^7_{\gamma,\delta,w} = \sum_{i \in O} {}^2D^2_{i,w} Y^4_{i,\gamma} Y^{2,*}_{i,\delta} \quad (3r_D r_T^2 N_o) \quad (11475)$$

$$\tau^8_{\gamma,\delta,w} = \sum_{\epsilon \in A} Z^*_{\epsilon,\delta} \tau^6_{\gamma,\epsilon,w} \tau^7_{\gamma,\epsilon,w} \quad (3r_D r_T^3) \quad (11476)$$

$$\tau^9_{\gamma,\delta,w} = \sum_{\epsilon \in A} Z_{\gamma,\epsilon} \tau^8_{\epsilon,\delta,w} \quad (2r_D r_T^3) \quad (11477)$$

$${}^2R^4_{i,\gamma} \leftarrow \sum_{\delta \in A} \sum_{w \in D} {}^2D^4_{i,w} Y^2_{i,\delta} \tau^5_{\delta,\gamma,w} \tau^9_{\delta,\gamma,w} \quad (4r_D r_T^2 N_o) \quad (11478)$$

Raw expression

$${}^2R^4_{j,\zeta} \leftarrow - \sum_{\gamma \in A} \sum_{i \in O} \sum_{k \in O} \sum_{a \in V} \sum_{b \in V} \sum_{c \in V} \sum_{d \in V} \frac{1}{2} {}^1T_{a,k} Y^{1,*}_{a,\gamma} Y^{2,*}_{i,\gamma} Z^*_{\gamma,\zeta} Y^{3,*}_{b,\zeta} {}^2D^{a,i,b,j} {}^2T_{c,i,d,j} V_{b,d,k,c} \quad (11479)$$

Factorized expression

$$\tau^0_{\gamma,\alpha,w} = \sum_{a \in V} {}^2D^3_{a,w} W^1_{a,\alpha} Y^{3,*}_{a,\gamma} \quad (3r_D r_T r_V N_v) \quad (11480)$$

$$\tau^1_{\gamma,\alpha} = \sum_{a \in V} W^2_{a,\alpha} Y^1_{a,\gamma} \quad (2r_T r_V N_v) \quad (11481)$$

$$\tau^2_{\gamma,\alpha,i} = \sum_{\delta \in A} Y^2_{i,\delta} Z_{\delta,\gamma} \tau^1_{\delta,\alpha} \quad (3r_T^2 r_V N_o) \quad (11482)$$

$$\tau^3_{\gamma,w,i} = \sum_{a \in V} {}^2D^1_{a,w} {}^1T_{a,i} Y^{1,*}_{a,\gamma} \quad (3r_D r_T N_o N_v) \quad (11483)$$

$$\tau^4_{\gamma,w,i,j} = \sum_{\delta \in A} Y^{2,*}_{j,\delta} Z^*_{\delta,\gamma} \tau^3_{\delta,w,i} \quad (3r_D r_T^2 N_o^2) \quad (11484)$$

$$\tau^5_{\gamma,\delta,w,i} = \sum_{j \in O} {}^2D^2_{j,w} Y^4_{j,\gamma} \tau^4_{\delta,w,i,j} \quad (3r_D r_T^2 N_o^2) \quad (11485)$$

$$\tau^6_{\gamma,\alpha} = \sum_{a \in V} W^4_{a,\alpha} Y^3_{a,\gamma} \quad (2r_T r_V N_v) \quad (11486)$$

$$\tau^7_{\gamma,\alpha,i} = \sum_{\beta \in B} X_{\alpha,\beta} W^3_{i,\beta} \tau^6_{\gamma,\beta} \quad (3r_T r_V^2 N_o) \quad (11487)$$

$$\tau^8_{\gamma,\delta,\alpha,w} = \sum_{i \in O} \tau^7_{\gamma,\alpha,i} \tau^5_{\gamma,\delta,w,i} \quad (2r_D r_T^2 r_V N_o) \quad (11488)$$

$$\tau^9_{\gamma,\alpha,w,i} = \sum_{\delta \in A} \tau^2_{\delta,\alpha,i} \tau^8_{\delta,\gamma,\alpha,w} \quad (2r_D r_T^2 r_V N_o) \quad (11489)$$

$$\tau^{10}_{\gamma,w,i} = \sum_{\alpha \in B} \tau^0_{\gamma,\alpha,w} \tau^9_{\gamma,\alpha,w,i} \quad (2r_D r_T r_V N_o) \quad (11490)$$

$${}^2R^4_{i,\gamma} \leftarrow - \sum_{w \in D} \frac{1}{2} {}^2D^4_{i,w} \tau^{10}_{\gamma,w,i} \quad (2r_D r_T N_o) \quad (11491)$$

Raw expression

$${}^2R^4_{j,\zeta} \leftarrow - \sum_{\gamma \in A} \sum_{i \in O} \sum_{k \in O} \sum_{a \in V} \sum_{b \in V} \sum_{c \in V} \sum_{d \in V} \frac{1}{2} {}^1T_{a,k} Y^{1,*}_{a,\gamma} Y^{2,*}_{i,\gamma} Z^*_{\gamma,\zeta} Y^{3,*}_{b,\zeta} {}^2D^{a,i,b,j} {}^2T_{c,j,d,i} V_{b,c,k,d} \quad (11492)$$

Factorized expression

$$\tau^0_{\gamma,\alpha,w} = \sum_{a \in V} {}^2D^3_{a,w} W^1_{a,\alpha} Y^{3,*}_{a,\gamma} \quad (3r_D r_T r_V N_v) \quad (11493)$$

$$\tau^1_{\gamma,\alpha} = \sum_{a \in V} W^2_{a,\alpha} Y^3_{a,\gamma} \quad (2r_T r_V N_v) \quad (11494)$$

$$\tau^2_{\gamma,\alpha,i} = \sum_{\delta \in A} Z_{\gamma,\delta} Y^4_{i,\delta} \tau^1_{\delta,\alpha} \quad (3r_T^2 r_V N_o) \quad (11495)$$

$$\tau^3_{\gamma,w,i} = \sum_{a \in V} {}^2D^1_{a,w} {}^1T_{a,i} Y^{1,*}_{a,\gamma} \quad (3r_D r_T N_o N_v) \quad (11496)$$

$$\tau^4_{\gamma,w,i,j} = \sum_{\delta \in A} Y^{2,*}_{j,\delta} Z^*_{\delta,\gamma} \tau^3_{\delta,w,i} \quad (3r_D r_T^2 N_o^2) \quad (11497)$$

$$\tau^5_{\gamma,\delta,w,i} = \sum_{j \in O} {}^2D^2_{j,w} Y^2_{j,\gamma} \tau^4_{\delta,w,i,j} \quad (3r_D r_T^2 N_o^2) \quad (11498)$$

$$\tau^6_{\gamma,\alpha} = \sum_{a \in V} W^4_{a,\alpha} Y^1_{a,\gamma} \quad (2r_T r_V N_v) \quad (11499)$$

$$\tau^7_{\gamma,\alpha,i} = \sum_{\beta \in B} X_{\alpha,\beta} W^3_{i,\beta} \tau^6_{\gamma,\beta} \quad (3r_T r_V^2 N_o) \quad (11500)$$

$$\tau^8_{\gamma,\delta,\alpha,w} = \sum_{i \in O} \tau^7_{\gamma,\alpha,i} \tau^5_{\gamma,\delta,w,i} \quad (2r_D r_T^2 r_V N_o) \quad (11501)$$

$$\tau^9_{\gamma,\alpha,w,i} = \sum_{\delta \in A} \tau^2_{\delta,\alpha,i} \tau^8_{\delta,\gamma,\alpha,w} \quad (2r_D r_T^2 r_V N_o) \quad (11502)$$

$$\tau^{10}_{\gamma,w,i} = \sum_{\alpha \in B} \tau^0_{\gamma,\alpha,w} \tau^9_{\gamma,\alpha,w,i} \quad (2r_D r_T r_V N_o) \quad (11503)$$

$${}^2R^4_{i,\gamma} \leftarrow - \sum_{w \in D} \frac{1}{2} {}^2D^4_{i,w} \tau^{10}_{\gamma,w,i} \quad (2r_D r_T N_o) \quad (11504)$$

Raw expression

$${}^2R^4_{j,\zeta} \leftarrow - \sum_{\gamma \in A} \sum_{i \in O} \sum_{k \in O} \sum_{a \in V} \sum_{b \in V} \sum_{c \in V} \sum_{d \in V} \frac{1}{2} {}^1T_{b,k} Y^{1,*}_{a,\gamma} Y^{2,*}_{i,\gamma} Z^*_{\gamma,\zeta} Y^{3,*}_{b,\zeta} {}^2D^{a,i,b,j} {}^2T_{c,i,d,j} V_{a,c,k,d} \quad (11505)$$

Factorized expression

$$\tau^0_{\gamma,w,i} = \sum_{a \in V} {}^2D^3_{a,w} {}^1T_{a,i} Y^{3,*}_{a,\gamma} \quad (3r_D r_T N_o N_v) \quad (11506)$$

$$\tau^1_{\gamma,\alpha,w} = \sum_{a \in V} {}^2D^1_{a,w} W^1_{a,\alpha} Y^{1,*}_{a,\gamma} \quad (3r_D r_T r_V N_v) \quad (11507)$$

$$\tau^2_{\gamma,\alpha} = \sum_{a \in V} W^2_{a,\alpha} Y^1_{a,\gamma} \quad (2r_T r_V N_v) \quad (11508)$$

$$\tau^3_{\gamma,\alpha,i} = \sum_{\delta \in A} Y^2_{i,\delta} Z_{\delta,\gamma} \tau^2_{\delta,\alpha} \quad (3r_T^2 r_V N_o) \quad (11509)$$

$$\tau^4_{\gamma,\delta,\alpha,w} = \sum_{i \in O} {}^2D^2_{i,w} Y^{2,*}_{i,\delta} \tau^1_{\delta,\alpha,w} \tau^3_{\gamma,\alpha,i} \quad (4r_D r_T^2 r_V N_o) \quad (11510)$$

$$\tau^5_{\gamma,\alpha} = \sum_{a \in V} W^4_{a,\alpha} Y^3_{a,\gamma} \quad (2r_T r_V N_v) \quad (11511)$$

$$\tau^6_{\gamma,\alpha,i} = \sum_{\beta \in B} X_{\alpha,\beta} W^3_{i,\beta} \tau^5_{\gamma,\beta} \quad (3r_T r_V^2 N_o) \quad (11512)$$

$$\tau^7_{\gamma,\delta,w,i} = \sum_{\alpha \in B} \tau^6_{\gamma,\alpha,i} \tau^4_{\gamma,\delta,\alpha,w} \quad (2r_D r_T^2 r_V N_o) \quad (11513)$$

$$\tau^8_{\gamma,w,i,j} = \sum_{\delta \in A} {}^2D^4_{i,w} Y^4_{i,\delta} \tau^7_{\delta,\gamma,w,j} \quad (3r_D r_T^2 N_o^2) \quad (11514)$$

$$\tau^9_{\gamma,\delta,i} = \sum_{w \in D} \sum_{j \in O} \tau^0_{\delta,w,j} \tau^8_{\gamma,w,i,j} \quad (2r_D r_T^2 N_o^2) \quad (11515)$$

$${}^2R^4_{i,\gamma} \leftarrow - \sum_{\delta \in A} \frac{1}{2} Z^*_{\delta,\gamma} \tau^9_{\delta,\gamma,i} \quad (2r_T^2 N_o) \quad (11516)$$

Raw expression

$${}^2R^4_{j,\zeta} \leftarrow - \sum_{\gamma \in A} \sum_{i \in O} \sum_{k \in O} \sum_{a \in V} \sum_{b \in V} \sum_{c \in V} \sum_{d \in V} \frac{1}{2} {}^1T_{b,k} Y^{1,*}_{a,\gamma} Y^{2,*}_{i,\gamma} Z^*_{\gamma,\zeta} Y^{3,*}_{b,\zeta} {}^2D^{a,i,b,j} {}^2T_{c,j,d,i} V_{a,d,k,c} \quad (11517)$$

Factorized expression

$$\tau^0_{\gamma,w,i} = \sum_{a \in V} {}^2D^3_{a,w} {}^1T_{a,i} Y^{3,*}_{a,\gamma} \quad (3r_D r_T N_o N_v) \quad (11518)$$

$$\tau^1_{\gamma,\alpha,w} = \sum_{a \in V} {}^2D^1_{a,w} W^1_{a,\alpha} Y^{1,*}_{a,\gamma} \quad (3r_D r_T r_V N_v) \quad (11519)$$

$$\tau^2_{\gamma,\alpha} = \sum_{a \in V} W^2_{a,\alpha} Y^3_{a,\gamma} \quad (2r_T r_V N_v) \quad (11520)$$

$$\tau^3_{\gamma,\alpha,i} = \sum_{\delta \in A} Z_{\gamma,\delta} Y^4_{i,\delta} \tau^2_{\delta,\alpha} \quad (3r_T^2 r_V N_o) \quad (11521)$$

$$\tau^4_{\gamma,\delta,\alpha,w} = \sum_{i \in O} {}^2D^2_{i,w} Y^{2,*}_{i,\delta} \tau^1_{\delta,\alpha,w} \tau^3_{\gamma,\alpha,i} \quad (4r_D r_T^2 r_V N_o) \quad (11522)$$

$$\tau^5_{\gamma,\alpha} = \sum_{a \in V} W^4_{a,\alpha} Y^1_{a,\gamma} \quad (2r_T r_V N_v) \quad (11523)$$

$$\tau^6_{\gamma,\alpha,i} = \sum_{\beta \in B} X_{\alpha,\beta} W^3_{i,\beta} \tau^5_{\gamma,\beta} \quad (3r_T r_V^2 N_o) \quad (11524)$$

$$\tau^7_{\gamma,\delta,w,i} = \sum_{\alpha \in B} \tau^6_{\gamma,\alpha,i} \tau^4_{\gamma,\delta,\alpha,w} \quad (2r_D r_T^2 r_V N_o) \quad (11525)$$

$$\tau^8_{\gamma,w,i,j} = \sum_{\delta \in A} {}^2D^4_{i,w} Y^2_{i,\delta} \tau^7_{\delta,\gamma,w,j} \quad (3r_D r_T^2 N_o^2) \quad (11526)$$

$$\tau^9_{\gamma,\delta,i} = \sum_{w \in D} \sum_{j \in O} \tau^0_{\delta,w,j} \tau^8_{\gamma,w,i,j} \quad (2r_D r_T^2 N_o^2) \quad (11527)$$

$${}^2R^4_{i,\gamma} \leftarrow - \sum_{\delta \in A} \frac{1}{2} Z^*_{\delta,\gamma} \tau^9_{\delta,\gamma,i} \quad (2r_T^2 N_o) \quad (11528)$$

Raw expression

$${}^2R^4_{j,\zeta} \leftarrow - \sum_{\gamma \in A} \sum_{i \in O} \sum_{k \in O} \sum_{a \in V} \sum_{b \in V} \sum_{c \in V} \sum_{d \in V} \frac{1}{2} {}^1T_{c,i} Y^{1,*}_{a,\gamma} Y^{2,*}_{i,\gamma} Z^*_{\gamma,\zeta} Y^{3,*}_{b,\zeta} {}^2D^{a,i,b,j} {}^2T_{a,k,d,j} V_{b,d,k,c} \quad (11529)$$

Factorized expression

$$\tau^0_{\gamma,\delta,w} = \sum_{a \in V} {}^2D^3_{a,w} Y^1_{a,\gamma} Y^{3,*}_{a,\delta} \quad (3r_D r_T^2 N_v) \quad (11530)$$

$$\tau^1_{\gamma,\alpha} = \sum_{i \in O} W^3_{i,\alpha} Y^2_{i,\gamma} \quad (2r_T r_V N_o) \quad (11531)$$

$$\tau^2_{\gamma,\alpha} = \sum_{a \in V} W^4_{a,\alpha} Y^3_{a,\gamma} \quad (2r_T r_V N_v) \quad (11532)$$

$$\tau^3_{\gamma,\alpha,i} = \sum_{\delta \in A} Z_{\gamma,\delta} Y^4_{i,\delta} \tau^2_{\delta,\alpha} \quad (3r_T^2 r_V N_o) \quad (11533)$$

$$\tau^4_{\alpha,i} = \sum_{a \in V} {}^1T_{a,i} W^2_{a,\alpha} \quad (2r_V N_o N_v) \quad (11534)$$

$$\tau^5_{\gamma,\alpha,w} = \sum_{i \in O} {}^2D^2_{i,w} Y^{2,*}_{i,\gamma} \tau^4_{\alpha,i} \quad (3r_D r_T r_V N_o) \quad (11535)$$

$$\tau^6_{\gamma,\alpha,w} = \sum_{a \in V} {}^2D^1_{a,w} W^1_{a,\alpha} Y^{1,*}_{a,\gamma} \quad (3r_D r_T r_V N_v) \quad (11536)$$

$$\tau^7_{\gamma,\alpha,w} = \sum_{\beta \in B} X_{\beta,\alpha} \tau^5_{\gamma,\beta,w} \tau^6_{\gamma,\beta,w} \quad (3r_D r_T r_V^2) \quad (11537)$$

$$\tau^8_{\gamma,\alpha,w} = \sum_{\delta \in A} Z^*_{\delta,\gamma} \tau^7_{\delta,\alpha,w} \quad (2r_D r_T^2 r_V) \quad (11538)$$

$$\tau^9_{\gamma,\delta,w,i} = \sum_{\alpha \in B} \tau^1_{\gamma,\alpha} \tau^3_{\gamma,\alpha,i} \tau^8_{\delta,\alpha,w} \quad (3r_D r_T^2 r_V N_o) \quad (11539)$$

$$\tau^{10}_{\gamma,w,i} = \sum_{\delta \in A} \tau^0_{\delta,\gamma,w} \tau^9_{\delta,\gamma,w,i} \quad (2r_D r_T^2 N_o) \quad (11540)$$

$${}^2R^4_{i,\gamma} \leftarrow - \sum_{w \in D} \frac{1}{2} {}^2D^4_{i,w} \tau^{10}_{\gamma,w,i} \quad (2r_D r_T N_o) \quad (11541)$$

Raw expression

$${}^2R^4_{j,\zeta} \leftarrow - \sum_{\gamma \in A} \sum_{i \in O} \sum_{k \in O} \sum_{a \in V} \sum_{b \in V} \sum_{c \in V} \sum_{d \in V} \frac{1}{2} {}^1T_{c,i} Y^{1,*}_{a,\gamma} Y^{2,*}_{i,\gamma} Z^*_{\gamma,\zeta} Y^{3,*}_{b,\zeta} {}^2D^{a,i,b,j} {}^2T_{b,j,d,k} V_{a,d,k,c} \quad (11542)$$

Factorized expression

$$\tau^0_{\gamma,\delta,w} = \sum_{a \in V} {}^2D^3_{a,w} Y^3_{a,\gamma} Y^{3,*}_{a,\delta} \quad (3r_D r_T^2 N_v) \quad (11543)$$

$$\tau^1_{\gamma,\alpha} = \sum_{a \in V} W^4_{a,\alpha} Y^1_{a,\gamma} \quad (2r_T r_V N_v) \quad (11544)$$

$$\tau^2_{\gamma,\alpha,i} = \sum_{\delta \in A} Y^2_{i,\delta} Z_{\delta,\gamma} \tau^1_{\delta,\alpha} \quad (3r_T^2 r_V N_o) \quad (11545)$$

$$\tau^3_{\gamma,\alpha} = \sum_{i \in O} W^3_{i,\alpha} Y^4_{i,\gamma} \quad (2r_T r_V N_o) \quad (11546)$$

$$\tau^4_{\alpha,i} = \sum_{a \in V} {}^1T_{a,i} W^2_{a,\alpha} \quad (2r_V N_o N_v) \quad (11547)$$

$$\tau^3_{\gamma,\alpha,i} = \sum_{j \in O} Y^4_{j,\gamma} \tau^2_{\alpha,i,j} \quad (2r_T r_V N_o^2) \quad (11559)$$

$$\tau^5_{\gamma,\alpha,w} = \sum_{i \in O} {}^2D^2_{i,w} Y^{2,*}_{i,\gamma} \tau^4_{\alpha,i} \quad (3r_D r_T r_V N_o) \quad (11548)$$

$$\tau^4_{\gamma,\alpha} = \sum_{a \in V} W^2_{a,\alpha} Y^3_{a,\gamma} \quad (2r_T r_V N_v) \quad (11560)$$

$$\tau^6_{\gamma,\alpha,w} = \sum_{a \in V} {}^2D^1_{a,w} W^1_{a,\alpha} Y^{1,*}_{a,\gamma} \quad (3r_D r_T r_V N_v) \quad (11549)$$

$$\tau^5_{\gamma,i,a} = \sum_{\alpha \in B} W^1_{a,\alpha} \tau^4_{\gamma,\alpha} \tau^3_{\gamma,\alpha,i} \quad (3r_T r_V N_o N_v) \quad (11561)$$

$$\tau^7_{\gamma,\alpha,w} = \sum_{\beta \in B} X_{\beta,\alpha} \tau^5_{\gamma,\beta,w} \tau^6_{\gamma,\beta,w} \quad (3r_D r_T r_V^2) \quad (11550)$$

$$\tau^6_{\gamma,\delta,w} = \sum_{i \in O} \sum_{a \in V} {}^2D^1_{a,w} {}^2D^2_{i,w} Y^{1,*}_{a,\delta} Y^{2,*}_{i,\delta} \tau^5_{\gamma,i,a} \quad (5r_D r_T^2 N_o N_v) \quad (11562)$$

$$\tau^8_{\gamma,\alpha,w} = \sum_{\delta \in A} Z^*_{\delta,\gamma} \tau^7_{\delta,\alpha,w} \quad (2r_D r_T^2 r_V) \quad (11551)$$

$$\tau^7_{\gamma,\delta,w} = \sum_{\epsilon \in A} Z^*_{\epsilon,\delta} \tau^6_{\gamma,\epsilon,w} \quad (2r_D r_T^3) \quad (11563)$$

$$\tau^9_{\gamma,\delta,w,i} = \sum_{\alpha \in B} \tau^3_{\gamma,\alpha} \tau^2_{\gamma,\alpha,i} \tau^8_{\delta,\alpha,w} \quad (3r_D r_T^2 r_V N_o) \quad (11552)$$

$$\tau^8_{\gamma,\delta,w} = \sum_{\epsilon \in A} Z_{\gamma,\epsilon} \tau^7_{\epsilon,\delta,w} \quad (2r_D r_T^3) \quad (11564)$$

$$\tau^{10}_{\gamma,w,i} = \sum_{\delta \in A} \tau^0_{\delta,\gamma,w} \tau^9_{\delta,\gamma,w,i} \quad (2r_D r_T^2 N_o) \quad (11553)$$

$${}^2R^4_{i,\gamma} \leftarrow - \sum_{\delta \in A} \sum_{w \in D} \frac{1}{2} {}^2D^4_{i,w} Y^2_{i,\delta} \tau^0_{\delta,\gamma,w} \tau^8_{\delta,\gamma,w} \quad (4r_D r_T^2 N_o) \quad (11565)$$

Raw expression

$${}^2R^4_{i,\gamma} \leftarrow - \sum_{w \in D} \frac{1}{2} {}^2D^4_{i,w} \tau^{10}_{\gamma,w,i} \quad (2r_D r_T N_o) \quad (11554)$$

$${}^2R^4_{j,\zeta} \leftarrow - \sum_{\gamma \in A} \sum_{i \in O} \sum_{k \in O} \sum_{a \in V} \sum_{b \in V} \sum_{c \in V} \sum_{d \in V} \frac{1}{2} {}^1T_{c,i} Y^{1,*}_{a,\gamma} Y^{2,*}_{i,\gamma} Z^*_{\gamma,\zeta} Y^{3,*}_{b,\zeta} {}^2D^{a,i,b,j} {}^2T_{d,j,a,k} V_{b,d,k,c} \quad (11566)$$

Raw expression

$${}^2R^4_{j,\zeta} \leftarrow - \sum_{\gamma \in A} \sum_{i \in O} \sum_{k \in O} \sum_{a \in V} \sum_{b \in V} \sum_{c \in V} \sum_{d \in V} \frac{1}{2} {}^1T_{c,i} Y^{1,*}_{a,\gamma} Y^{2,*}_{i,\gamma} Z^*_{\gamma,\zeta} Y^{3,*}_{b,\zeta} {}^2D^{a,i,b,j} {}^2T_{b,k,d,j} V_{a,c,k,d} \quad (11555)$$

Factorized expression

Factorized expression

$$\tau^0_{\gamma,\delta,w} = \sum_{a \in V} {}^2D^3_{a,w} Y^1_{a,\gamma} Y^{3,*}_{a,\delta} \quad (3r_D r_T^2 N_v) \quad (11556)$$

$$\tau^0_{\gamma,\delta,w} = \sum_{a \in V} {}^2D^3_{a,w} Y^3_{a,\gamma} Y^{3,*}_{a,\delta} \quad (3r_D r_T^2 N_v) \quad (11567)$$

$$\tau^1_{\alpha,i} = \sum_{a \in V} {}^1T_{a,i} W^4_{a,\alpha} \quad (2r_V N_o N_v) \quad (11557)$$

$$\tau^1_{\alpha,i} = \sum_{a \in V} {}^1T_{a,i} W^4_{a,\alpha} \quad (2r_V N_o N_v) \quad (11568)$$

$$\tau^2_{\alpha,i,j} = \sum_{\beta \in B} X_{\alpha,\beta} W^3_{j,\beta} \tau^1_{\beta,i} \quad (3r_V^2 N_o^2) \quad (11558)$$

$$\tau^2_{\alpha,i,j} = \sum_{\beta \in B} X_{\alpha,\beta} W^3_{j,\beta} \tau^1_{\beta,i} \quad (3r_V^2 N_o^2) \quad (11569)$$

$$\tau^3_{\gamma,\alpha,i} = \sum_{j \in O} Y^2_{j,\gamma} \tau^2_{\alpha,i,j} \quad (2r_T r_V N_o^2) \quad (11570)$$

$$\tau^3_{\gamma,\alpha,i} = \sum_{j \in O} Y^2_{j,\gamma} \tau^2_{\alpha,i,j} \quad (2r_T r_V N_o^2) \quad (11570)$$



$$\tau^4_{\gamma,\alpha} = \sum_{a \in V} W^2_{a,\alpha} Y^1_{a,\gamma} \quad (2r_T r_V N_v) \quad (11571)$$

$$\tau^5_{\alpha,i} = \sum_{a \in V} {}^1T_{a,i} W^4_{a,\alpha} \quad (2r_V N_o N_v) \quad (11583)$$

$$\tau^5_{\gamma,i,a} = \sum_{\alpha \in B} W^1_{a,\alpha} \tau^4_{\gamma,\alpha} \tau^3_{\gamma,\alpha,i} \quad (3r_T r_V N_o N_v) \quad (11572)$$

$$\tau^6_{\alpha,i,j} = \sum_{\beta \in B} X_{\alpha,\beta} W^3_{j,\beta} \tau^5_{\beta,i} \quad (3r_V^2 N_o^2) \quad (11584)$$

$$\tau^6_{\gamma,\delta,w} = \sum_{i \in O} \sum_{a \in V} {}^2D^1_{a,w} {}^2D^2_{i,w} Y^{1,*}_{a,\delta} Y^{2,*}_{i,\delta} \tau^5_{\gamma,i,a} \quad (5r_D r_T^2 N_o N_v) \quad (11573)$$

$$\tau^7_{\gamma,\alpha,i} = \sum_{j \in O} Y^2_{j,\gamma} \tau^6_{\alpha,i,j} \quad (2r_T r_V N_o^2) \quad (11585)$$

$$\tau^7_{\gamma,\delta,w} = \sum_{\epsilon \in A} Z^*_{\epsilon,\delta} \tau^6_{\gamma,\epsilon,w} \quad (2r_D r_T^3) \quad (11574)$$

$$\tau^8_{\gamma,\delta,\alpha,w} = \sum_{i \in O} \tau^7_{\gamma,\alpha,i} \tau^4_{\gamma,\delta,w,i} \quad (2r_D r_T^2 r_V N_o) \quad (11586)$$

$$\tau^9_{\gamma,\alpha,w,i} = \sum_{\delta \in A} \tau^2_{\delta,\alpha,i} \tau^8_{\delta,\gamma,\alpha,w} \quad (2r_D r_T^2 r_V N_o) \quad (11587)$$

$$\tau^8_{\gamma,\delta,w} = \sum_{\epsilon \in A} Z_{\epsilon,\gamma} \tau^7_{\epsilon,\delta,w} \quad (2r_D r_T^3) \quad (11575)$$

$$\tau^{10}_{\gamma,w,i} = \sum_{\alpha \in B} \tau^0_{\gamma,\alpha,w} \tau^9_{\gamma,\alpha,w,i} \quad (2r_D r_T r_V N_o) \quad (11588)$$

$${}^2R^4_{i,\gamma} \leftarrow - \sum_{\delta \in A} \sum_{w \in D} \frac{1}{2} {}^2D^4_{i,w} Y^4_{i,\delta} \tau^0_{\delta,\gamma,w} \tau^8_{\delta,\gamma,w} \quad (4r_D r_T^2 N_o) \quad (11576)$$

$${}^2R^4_{i,\gamma} \leftarrow - \sum_{w \in D} \frac{1}{2} {}^2D^4_{i,w} \tau^{10}_{\gamma,w,i} \quad (2r_D r_T N_o) \quad (11589)$$

Raw expression

$${}^2R^4_{j,\zeta} \leftarrow - \sum_{\gamma \in A} \sum_{i \in O} \sum_{k \in O} \sum_{a \in V} \sum_{b \in V} \sum_{c \in V} \sum_{d \in V} \frac{1}{2} {}^1T_{c,i} Y^{1,*}_{a,\gamma} Y^{2,*}_{i,\gamma} Z^*_{\gamma,\zeta} Y^{3,*}_{b,\zeta} {}^2D^{a,i,b,j} {}^2T_{d,j,b,k} V_{a,c,k,d} \quad (11577)$$

Raw expression

$${}^2R^4_{j,\zeta} \leftarrow - \sum_{\gamma \in A} \sum_{i \in O} \sum_{k \in O} \sum_{a \in V} \sum_{b \in V} \sum_{c \in V} \sum_{d \in V} \frac{1}{2} {}^1T_{c,i} Y^{1,*}_{a,\gamma} Y^{2,*}_{i,\gamma} Z^*_{\gamma,\zeta} Y^{3,*}_{b,\zeta} {}^2D^{a,i,b,j} {}^2T_{d,k,b,j} V_{a,d,k,c} \quad (11590)$$

Factorized expression

$$\tau^0_{\gamma,\alpha,w} = \sum_{a \in V} {}^2D^3_{a,w} W^1_{a,\alpha} Y^{3,*}_{a,\gamma} \quad (3r_D r_T r_V N_v) \quad (11578)$$

Factorized expression

$$\tau^0_{\gamma,\alpha,w} = \sum_{a \in V} {}^2D^3_{a,w} W^1_{a,\alpha} Y^{3,*}_{a,\gamma} \quad (3r_D r_T r_V N_v) \quad (11591)$$

$$\tau^1_{\gamma,\alpha} = \sum_{a \in V} W^2_{a,\alpha} Y^3_{a,\gamma} \quad (2r_T r_V N_v) \quad (11579)$$

$$\tau^1_{\gamma,\alpha} = \sum_{a \in V} W^2_{a,\alpha} Y^1_{a,\gamma} \quad (2r_T r_V N_v) \quad (11592)$$

$$\tau^2_{\gamma,\alpha,i} = \sum_{\delta \in A} Z_{\gamma,\delta} Y^4_{i,\delta} \tau^1_{\delta,\alpha} \quad (3r_T^2 r_V N_o) \quad (11580)$$

$$\tau^2_{\gamma,\alpha,i} = \sum_{\delta \in A} Y^2_{i,\delta} Z_{\delta,\gamma} \tau^1_{\delta,\alpha} \quad (3r_T^2 r_V N_o) \quad (11593)$$

$$\tau^3_{\gamma,\delta,w} = \sum_{a \in V} {}^2D^1_{a,w} Y^1_{a,\gamma} Y^{1,*}_{a,\delta} \quad (3r_D r_T^2 N_v) \quad (11581)$$

$$\tau^3_{\gamma,\delta,w} = \sum_{a \in V} {}^2D^1_{a,w} Y^3_{a,\gamma} Y^{1,*}_{a,\delta} \quad (3r_D r_T^2 N_v) \quad (11594)$$

$$\tau^4_{\gamma,\delta,w,i} = \sum_{\epsilon \in A} {}^2D^2_{i,w} Y^{2,*}_{i,\epsilon} Z^*_{\epsilon,\delta} \tau^3_{\gamma,\epsilon,w} \quad (4r_D r_T^3 N_o) \quad (11582)$$

$$\tau^4_{\gamma,\delta,w,i} = \sum_{\epsilon \in A} {}^2D^2_{i,w} Y^{2,*}_{i,\epsilon} Z^*_{\epsilon,\delta} \tau^3_{\gamma,\epsilon,w} \quad (4r_D r_T^3 N_o) \quad (11595)$$

$$\tau^5_{\alpha,i} = \sum_{a \in V} {}^1T_{a,i} W^4_{a,\alpha} \quad (2r_V N_o N_v) \quad (11596)$$

$$\tau^6_{\alpha,i,j} = \sum_{\beta \in B} X_{\alpha,\beta} W^3_{j,\beta} \tau^5_{\beta,i} \quad (3r_V^2 N_o^2) \quad (11597)$$

$$\tau^7_{\gamma,\alpha,i} = \sum_{j \in O} Y^4_{j,\gamma} \tau^6_{\alpha,i,j} \quad (2r_T r_V N_o^2) \quad (11598)$$

$$\tau^8_{\gamma,\delta,\alpha,w} = \sum_{i \in O} \tau^7_{\gamma,\alpha,i} \tau^4_{\gamma,\delta,w,i} \quad (2r_D r_T^2 r_V N_o) \quad (11599)$$

$$\tau^9_{\gamma,\alpha,w,i} = \sum_{\delta \in A} \tau^2_{\delta,\alpha,i} \tau^8_{\delta,\gamma,\alpha,w} \quad (2r_D r_T^2 r_V N_o) \quad (11600)$$

$$\tau^{10}_{\gamma,w,i} = \sum_{\alpha \in B} \tau^0_{\gamma,\alpha,w} \tau^9_{\gamma,\alpha,w,i} \quad (2r_D r_T r_V N_o) \quad (11601)$$

$${}^2R^4_{i,\gamma} \leftarrow - \sum_{w \in D} \frac{1}{2} {}^2D^4_{i,w} \tau^{10}_{\gamma,w,i} \quad (2r_D r_T N_o) \quad (11602)$$

Raw expression

$${}^2R^4_{j,\zeta} \leftarrow - \sum_{\gamma \in A} \sum_{i \in O} \sum_{k \in O} \sum_{a \in V} \sum_{b \in V} \sum_{c \in V} \sum_{d \in V} \frac{1}{2} {}^1T_{c,j} Y^{1,*}_{a,\gamma} Y^{2,*}_{i,\gamma} Z^*_{\gamma,\zeta} Y^{3,*}_{b,\zeta} {}^2D^{a,i,b,j} {}^2T_{a,i,d,k} V_{b,d,k,c} \quad (11603)$$

Factorized expression

$$\tau^0_{\gamma,\delta,w} = \sum_{a \in V} {}^2D^3_{a,w} Y^1_{a,\gamma} Y^{3,*}_{a,\delta} \quad (3r_D r_T^2 N_v) \quad (11604)$$

$$\tau^1_{\gamma,\alpha,w} = \sum_{a \in V} {}^2D^1_{a,w} W^1_{a,\alpha} Y^{1,*}_{a,\gamma} \quad (3r_D r_T r_V N_v) \quad (11605)$$

$$\tau^2_{\gamma,\alpha} = \sum_{a \in V} W^2_{a,\alpha} Y^3_{a,\gamma} \quad (2r_T r_V N_v) \quad (11606)$$

$$\tau^3_{\gamma,\alpha,i} = \sum_{\delta \in A} Z_{\gamma,\delta} Y^4_{i,\delta} \tau^2_{\delta,\alpha} \quad (3r_T^2 r_V N_o) \quad (11607)$$

$$\tau^4_{\gamma,\delta,\alpha,w} = \sum_{i \in O} {}^2D^2_{i,w} Y^{2,*}_{i,\delta} \tau^1_{\delta,\alpha,w} \tau^3_{\gamma,\alpha,i} \quad (4r_D r_T^2 r_V N_o) \quad (11608)$$

$$\tau^5_{\alpha,i} = \sum_{a \in V} {}^1T_{a,i} W^4_{a,\alpha} \quad (2r_V N_o N_v) \quad (11609)$$

$$\tau^6_{\alpha,i,j} = \sum_{\beta \in B} X_{\alpha,\beta} W^3_{j,\beta} \tau^5_{\beta,i} \quad (3r_V^2 N_o^2) \quad (11610)$$

$$\tau^7_{\gamma,\alpha,i} = \sum_{j \in O} Y^2_{j,\gamma} \tau^6_{\alpha,i,j} \quad (2r_T r_V N_o^2) \quad (11611)$$

$$\tau^8_{\gamma,\delta,w,i} = \sum_{\alpha \in B} \tau^7_{\gamma,\alpha,i} \tau^4_{\gamma,\delta,\alpha,w} \quad (2r_D r_T^2 r_V N_o) \quad (11612)$$

$$\tau^9_{\gamma,\delta,i} = \sum_{\epsilon \in A} \sum_{w \in D} {}^2D^4_{i,w} \tau^0_{\epsilon,\delta,w} \tau^8_{\epsilon,\gamma,w,i} \quad (3r_D r_T^3 N_o) \quad (11613)$$

$${}^2R^4_{i,\gamma} \leftarrow - \sum_{\delta \in A} \frac{1}{2} Z^*_{\delta,\gamma} \tau^9_{\delta,\gamma,i} \quad (2r_T^2 N_o) \quad (11614)$$

Raw expression

$${}^2R^4_{j,\zeta} \leftarrow - \sum_{\gamma \in A} \sum_{i \in O} \sum_{k \in O} \sum_{a \in V} \sum_{b \in V} \sum_{c \in V} \sum_{d \in V} \frac{1}{2} {}^1T_{c,j} Y^{1,*}_{a,\gamma} Y^{2,*}_{i,\gamma} Z^*_{\gamma,\zeta} Y^{3,*}_{b,\zeta} {}^2D^{a,i,b,j} {}^2T_{a,k,d,i} V_{b,c,k,d} \quad (11615)$$

Factorized expression

$$\tau^0_{\gamma,\delta,w} = \sum_{a \in V} {}^2D^3_{a,w} Y^3_{a,\gamma} Y^{3,*}_{a,\delta} \quad (3r_D r_T^2 N_v) \quad (11616)$$

$$\tau^1_{\gamma,\alpha,w} = \sum_{a \in V} {}^2D^1_{a,w} W^1_{a,\alpha} Y^{1,*}_{a,\gamma} \quad (3r_D r_T r_V N_v) \quad (11617)$$

$$\tau^2_{\gamma,\alpha} = \sum_{a \in V} W^2_{a,\alpha} Y^1_{a,\gamma} \quad (2r_T r_V N_v) \quad (11618)$$

$$\tau^3_{\gamma,\alpha,i} = \sum_{\delta \in A} Y^2_{i,\delta} Z_{\delta,\gamma} \tau^2_{\delta,\alpha} \quad (3r_T^2 r_V N_o) \quad (11619)$$

$$\tau^4_{\gamma,\delta,\alpha,w} = \sum_{i \in O} {}^2D^2_{i,w} Y^{2,*}_{i,\delta} \tau^1_{\delta,\alpha,w} \tau^3_{\gamma,\alpha,i} \quad (4r_D r_T^2 r_V N_o) \quad (11620)$$

$$\tau^5_{\alpha,i} = \sum_{a \in V} {}^1T_{a,i} W^4_{a,\alpha} \quad (2r_V N_o N_v) \quad (11621)$$

$$\tau^5_{\gamma,\alpha,w} = \sum_{\delta \in A} \sum_{i \in O} {}^2D^2_{i,w} Y^{2,*}_{i,\gamma} \tau^2_{\delta,\alpha} \tau^1_{\delta,\gamma,w} \tau^4_{\delta,\alpha,i} \quad (5r_D r_T^2 r_V N_o) \quad (11633)$$

$$\tau^6_{\alpha,i,j} = \sum_{\beta \in B} X_{\alpha,\beta} W^3_{j,\beta} \tau^5_{\beta,i} \quad (3r_V^2 N_o^2) \quad (11622)$$

$$\tau^6_{\gamma,\alpha,w} = \sum_{\beta \in B} X_{\alpha,\beta} \tau^5_{\gamma,\beta,w} \quad (2r_D r_T r_V^2) \quad (11634)$$

$$\tau^7_{\gamma,\alpha,i} = \sum_{j \in O} Y^4_{j,\gamma} \tau^6_{\alpha,i,j} \quad (2r_T r_V N_o^2) \quad (11623)$$

$$\tau^7_{\gamma,\alpha,w} = \sum_{\delta \in A} Z^*_{\delta,\gamma} \tau^6_{\delta,\alpha,w} \quad (2r_D r_T^2 r_V) \quad (11635)$$

$$\tau^8_{\gamma,\delta,w,i} = \sum_{\alpha \in B} \tau^7_{\gamma,\alpha,i} \tau^4_{\gamma,\delta,\alpha,w} \quad (2r_D r_T^2 r_V N_o) \quad (11624)$$

$$\tau^8_{\alpha,i} = \sum_{a \in V} {}^1T_{a,i} W^2_{a,\alpha} \quad (2r_V N_o N_v) \quad (11636)$$

$$\tau^9_{\gamma,\delta,i} = \sum_{\epsilon \in A} \sum_{w \in D} {}^2D^4_{i,w} \tau^0_{\epsilon,\delta,w} \tau^8_{\epsilon,\gamma,w,i} \quad (3r_D r_T^3 N_o) \quad (11625)$$

$$\tau^9_{\gamma,w,i} = \sum_{\alpha \in B} \tau^8_{\alpha,i} \tau^0_{\gamma,\alpha,w} \tau^7_{\gamma,\alpha,w} \quad (3r_D r_T r_V N_o) \quad (11637)$$

$${}^2R^4_{i,\gamma} \leftarrow - \sum_{\delta \in A} \frac{1}{2} Z^*_{\delta,\gamma} \tau^9_{\delta,\gamma,i} \quad (2r_T^2 N_o) \quad (11626)$$

$${}^2R^4_{i,\gamma} \leftarrow - \sum_{w \in D} \frac{1}{2} {}^2D^4_{i,w} \tau^9_{\gamma,w,i} \quad (2r_D r_T N_o) \quad (11638)$$

Raw expression

$${}^2R^4_{j,\zeta} \leftarrow - \sum_{\gamma \in A} \sum_{i \in O} \sum_{k \in O} \sum_{a \in V} \sum_{b \in V} \sum_{c \in V} \sum_{d \in V} \frac{1}{2} {}^1T_{c,j} Y^{1,*}_{a,\gamma} Y^{2,*}_{i,\gamma} Z^*_{\gamma,\zeta} Y^{3,*}_{b,\zeta} {}^2D^{a,i,b,j} {}^2T_{b,k,d,i} V_{a,d,k,c} \quad (11627)$$

Raw expression

$${}^2R^4_{j,\zeta} \leftarrow - \sum_{\gamma \in A} \sum_{i \in O} \sum_{k \in O} \sum_{a \in V} \sum_{b \in V} \sum_{c \in V} \sum_{d \in V} \frac{1}{2} {}^1T_{c,j} Y^{1,*}_{a,\gamma} Y^{2,*}_{i,\gamma} Z^*_{\gamma,\zeta} Y^{3,*}_{b,\zeta} {}^2D^{a,i,b,j} {}^2T_{d,i,a,k} V_{b,c,k,d} \quad (11639)$$

Factorized expression

$$\tau^0_{\gamma,\alpha,w} = \sum_{a \in V} {}^2D^3_{a,w} W^1_{a,\alpha} Y^{3,*}_{a,\gamma} \quad (3r_D r_T r_V N_v) \quad (11628)$$

Factorized expression

$$\tau^0_{\gamma,\alpha,w} = \sum_{a \in V} {}^2D^3_{a,w} W^1_{a,\alpha} Y^{3,*}_{a,\gamma} \quad (3r_D r_T r_V N_v) \quad (11640)$$

$$\tau^1_{\gamma,\delta,w} = \sum_{a \in V} {}^2D^1_{a,w} Y^1_{a,\gamma} Y^{1,*}_{a,\delta} \quad (3r_D r_T^2 N_v) \quad (11629)$$

$$\tau^1_{\gamma,\delta,w} = \sum_{a \in V} {}^2D^1_{a,w} Y^3_{a,\gamma} Y^{1,*}_{a,\delta} \quad (3r_D r_T^2 N_v) \quad (11641)$$

$$\tau^2_{\gamma,\alpha} = \sum_{i \in O} W^3_{i,\alpha} Y^2_{i,\gamma} \quad (2r_T r_V N_o) \quad (11630)$$

$$\tau^2_{\gamma,\alpha} = \sum_{a \in V} W^4_{a,\alpha} Y^1_{a,\gamma} \quad (2r_T r_V N_v) \quad (11642)$$

$$\tau^3_{\gamma,\alpha} = \sum_{a \in V} W^4_{a,\alpha} Y^3_{a,\gamma} \quad (2r_T r_V N_v) \quad (11631)$$

$$\tau^3_{\gamma,\alpha,i} = \sum_{\delta \in A} Y^2_{i,\delta} Z_{\delta,\gamma} \tau^2_{\delta,\alpha} \quad (3r_T^2 r_V N_o) \quad (11643)$$

$$\tau^4_{\gamma,\alpha,i} = \sum_{\delta \in A} Z_{\gamma,\delta} Y^4_{i,\delta} \tau^3_{\delta,\alpha} \quad (3r_T^2 r_V N_o) \quad (11632)$$

$$\tau^4_{\gamma,\alpha} = \sum_{i \in O} W^3_{i,\alpha} Y^4_{i,\gamma} \quad (2r_T r_V N_o) \quad (11644)$$

$$\tau^5_{\gamma,\alpha,w} = \sum_{\delta \in A} \sum_{i \in O} {}^2D^2_{i,w} Y^{2,*}_{i,\gamma} \tau^4_{\delta,\alpha} \tau^1_{\delta,\gamma,w} \tau^3_{\delta,\alpha,i} \quad (5r_D r_T^2 r_V \mathbb{A}_\alpha^6)_{\delta,w} = \sum_{i \in O} {}^2D^2_{i,w} Y^2_{i,\gamma} Y^{2,*}_{i,\delta} \quad (3r_D r_T^2 N_o) \quad (11658)$$

$$\tau^6_{\gamma,\alpha,w} = \sum_{\beta \in B} X_{\alpha,\beta} \tau^5_{\gamma,\beta,w} \quad (2r_D r_T r_V^2) \quad (11646)$$

$$\tau^7_{\gamma,\alpha,w} = \sum_{\delta \in A} Z^*_{\delta,\gamma} \tau^6_{\delta,\alpha,w} \quad (2r_D r_T^2 r_V) \quad (11647)$$

$$\tau^8_{\alpha,i} = \sum_{a \in V} {}^1T_{a,i} W^2_{a,\alpha} \quad (2r_V N_o N_v) \quad (11648)$$

$$\tau^9_{\gamma,w,i} = \sum_{\alpha \in B} \tau^8_{\alpha,i} \tau^0_{\gamma,\alpha,w} \tau^7_{\gamma,\alpha,w} \quad (3r_D r_T r_V N_o) \quad (11649)$$

$${}^2R^4_{i,\gamma} \leftarrow - \sum_{w \in D} \frac{1}{2} {}^2D^4_{i,w} \tau^9_{\gamma,w,i} \quad (2r_D r_T N_o) \quad (11650)$$

Raw expression

$${}^2R^4_{j,\zeta} \leftarrow - \sum_{\gamma \in A} \sum_{i \in O} \sum_{k \in O} \sum_{a \in V} \sum_{b \in V} \sum_{c \in V} \sum_{d \in V} \frac{1}{2} {}^1T_{c,j} Y^{1,*}_{a,\gamma} Y^{2,*}_{i,\gamma} Z^*_{\gamma,\zeta} Y^{3,*}_{b,\zeta} {}^2D^{a,i,b,j} {}^2T_{d,i,b,k} V_{a,d,k,c} \quad (11651)$$

Factorized expression

$$\tau^0_{\alpha,i} = \sum_{a \in V} {}^1T_{a,i} W^4_{a,\alpha} \quad (2r_V N_o N_v) \quad (11652)$$

$$\tau^1_{\alpha,i,j} = \sum_{\beta \in B} X_{\alpha,\beta} W^3_{j,\beta} \tau^0_{\beta,i} \quad (3r_V^2 N_o^2) \quad (11653)$$

$$\tau^2_{\gamma,\alpha,i} = \sum_{j \in O} Y^4_{j,\gamma} \tau^1_{\alpha,i,j} \quad (2r_T r_V N_o^2) \quad (11654)$$

$$\tau^3_{\gamma,\alpha} = \sum_{a \in V} W^2_{a,\alpha} Y^3_{a,\gamma} \quad (2r_T r_V N_v) \quad (11655)$$

$$\tau^4_{\gamma,i,a} = \sum_{\alpha \in B} W^1_{a,\alpha} \tau^3_{\gamma,\alpha} \tau^2_{\gamma,\alpha,i} \quad (3r_T r_V N_o N_v) \quad (11656)$$

$$\tau^5_{\gamma,\delta,w} = \sum_{a \in V} {}^2D^1_{a,w} Y^1_{a,\gamma} Y^{1,*}_{a,\delta} \quad (3r_D r_T^2 N_v) \quad (11657)$$

$$\tau^7_{\gamma,\delta,w} = \sum_{\epsilon \in A} Z^*_{\epsilon,\delta} \tau^5_{\gamma,\epsilon,w} \tau^6_{\gamma,\epsilon,w} \quad (3r_D r_T^3) \quad (11659)$$

$$\tau^8_{\gamma,\delta,w} = \sum_{\epsilon \in A} Z_{\epsilon,\gamma} \tau^7_{\epsilon,\delta,w} \quad (2r_D r_T^3) \quad (11660)$$

$$\tau^9_{\gamma,i,a} = \sum_{\delta \in A} \sum_{w \in D} {}^2D^3_{a,w} {}^2D^4_{i,w} \tau^4_{\delta,i,a} \tau^8_{\delta,\gamma,w} \quad (4r_D r_T^2 N_o N_v) \quad (11661)$$

$${}^2R^4_{i,\gamma} \leftarrow - \sum_{a \in V} \frac{1}{2} Y^{3,*}_{a,\gamma} \tau^9_{\gamma,i,a} \quad (2r_T N_o N_v) \quad (11662)$$

Raw expression

$${}^2R^4_{j,\zeta} \leftarrow - \sum_{\gamma \in A} \sum_{i \in O} \sum_{k \in O} \sum_{a \in V} \sum_{b \in V} \sum_{c \in V} \sum_{d \in V} \frac{1}{2} {}^1T_{c,j} Y^{1,*}_{a,\gamma} Y^{2,*}_{i,\gamma} Z^*_{\gamma,\zeta} Y^{3,*}_{b,\zeta} {}^2D^{a,i,b,j} {}^2T_{d,k,a,i} V_{b,d,k,c} \quad (11663)$$

Factorized expression

$$\tau^0_{\alpha,i} = \sum_{a \in V} {}^1T_{a,i} W^4_{a,\alpha} \quad (2r_V N_o N_v) \quad (11664)$$

$$\tau^1_{\alpha,i,j} = \sum_{\beta \in B} X_{\alpha,\beta} W^3_{j,\beta} \tau^0_{\beta,i} \quad (3r_V^2 N_o^2) \quad (11665)$$

$$\tau^2_{\gamma,\alpha,i} = \sum_{j \in O} Y^2_{j,\gamma} \tau^1_{\alpha,i,j} \quad (2r_T r_V N_o^2) \quad (11666)$$

$$\tau^3_{\gamma,\alpha} = \sum_{a \in V} W^2_{a,\alpha} Y^1_{a,\gamma} \quad (2r_T r_V N_v) \quad (11667)$$

$$\tau^4_{\gamma,i,a} = \sum_{\alpha \in B} W^1_{a,\alpha} \tau^3_{\gamma,\alpha} \tau^2_{\gamma,\alpha,i} \quad (3r_T r_V N_o N_v) \quad (11668)$$

$$\tau^5_{\gamma,\delta,w} = \sum_{a \in V} {}^2D^1_{a,w} Y^3_{a,\gamma} Y^{1,*}_{a,\delta} \quad (3r_D r_T^2 N_v) \quad (11669)$$

$$\tau^6_{\gamma,\delta,w} = \sum_{i \in O} {}^2D^2_{i,w} Y^4_{i,\gamma} Y^{2,*}_{i,\delta} \quad (3r_D r_T^2 N_o) \quad (11670)$$

$$\tau_{\gamma,\delta,w}^7 = \sum_{\epsilon \in A} Z_{\epsilon,\delta}^* \tau_{\gamma,\epsilon,w}^5 \tau_{\gamma,\epsilon,w}^6 \quad (3r_D r_T^3) \quad (11671)$$

$$\tau_{\gamma,\delta,w}^8 = \sum_{\epsilon \in A} Z_{\epsilon,\delta}^* \tau_{\gamma,\epsilon,w}^1 \tau_{\gamma,\epsilon,w}^7 \quad (3r_D r_T^3) \quad (11684)$$

$$\tau_{\gamma,\delta,w}^8 = \sum_{\epsilon \in A} Z_{\gamma,\epsilon} \tau_{\epsilon,\delta,w}^7 \quad (2r_D r_T^3) \quad (11672)$$

$$\tau_{\gamma,\delta,w}^9 = \sum_{\epsilon \in A} Z_{\gamma,\epsilon} \tau_{\epsilon,\delta,w}^8 \quad (2r_D r_T^3) \quad (11685)$$

$$\tau_{\gamma,i,a}^9 = \sum_{\delta \in A} \sum_{w \in D} {}^2D_{a,w}^3 {}^2D_{i,w}^4 \tau_{\delta,i,a}^4 \tau_{\delta,\gamma,w}^8 \quad (4r_D r_T^2 N_o N_v) {}^2R_{i,\gamma}^4 \leftarrow - \sum_{\delta \in A} \sum_{w \in D} \frac{1}{2} {}^2D_{i,w}^4 Y_{i,\delta}^2 \tau_{\delta,\gamma,w}^0 \tau_{\delta,\gamma,w}^9 \quad (4r_D r_T^2 N_o) \quad (11673) \quad (11686)$$

$${}^2R_{i,\gamma}^4 \leftarrow - \sum_{a \in V} \frac{1}{2} Y_{a,\gamma}^{3,*} \tau_{\gamma,i,a}^9 \quad (2r_T N_o N_v) \quad (11674)$$

Raw expression

$${}^2R_{j,\zeta}^4 \leftarrow - \sum_{\gamma \in A} \sum_{i \in O} \sum_{k \in O} \sum_{a \in V} \sum_{b \in V} \sum_{c \in V} \sum_{d \in V} \frac{1}{2} {}^1T_{c,k} Y_{a,\gamma}^{1,*} Y_{i,\gamma}^{2,*} Z_{\gamma,\zeta}^* Y_{b,\zeta}^{3,*} {}^2D_{a,i,b,j} {}^2T_{a,i,d,j} V_{b,c,k,d} \quad (11675)$$

Factorized expression

$$\tau_{\gamma,\delta,w}^0 = \sum_{a \in V} {}^2D_{a,w}^3 Y_{a,\gamma}^1 Y_{a,\delta}^{3,*} \quad (3r_D r_T^2 N_v) \quad (11676)$$

$$\tau_{\gamma,\delta,w}^1 = \sum_{i \in O} {}^2D_{i,w}^2 Y_{i,\gamma}^4 Y_{i,\delta}^{2,*} \quad (3r_D r_T^2 N_o) \quad (11677)$$

$$\tau_{\alpha,i}^2 = \sum_{a \in V} {}^1T_{a,i} W_{a,\alpha}^2 \quad (2r_V N_o N_v) \quad (11678)$$

$$\tau_{\alpha,\beta}^3 = \sum_{i \in O} W_{i,\beta}^3 \tau_{\alpha,i}^2 \quad (2r_V^2 N_o) \quad (11679)$$

$$\tau_{\alpha,a}^4 = \sum_{\beta \in B} X_{\alpha,\beta} W_{a,\beta}^4 \tau_{\alpha,\beta}^3 \quad (3r_V^2 N_v) \quad (11680)$$

$$\tau_{a,b}^5 = \sum_{\alpha \in B} W_{a,\alpha}^1 \tau_{\alpha,b}^4 \quad (2r_V N_v^2) \quad (11681)$$

$$\tau_{\gamma,a}^6 = \sum_{b \in V} Y_{b,\gamma}^3 \tau_{a,b}^5 \quad (2r_T N_v^2) \quad (11682)$$

$$\tau_{\gamma,\delta,w}^7 = \sum_{a \in V} {}^2D_{a,w}^1 Y_{a,w}^{1,*} \tau_{\gamma,a}^6 \quad (3r_D r_T^2 N_v) \quad (11683)$$

Raw expression

$${}^2R_{j,\zeta}^4 \leftarrow - \sum_{\gamma \in A} \sum_{i \in O} \sum_{k \in O} \sum_{a \in V} \sum_{b \in V} \sum_{c \in V} \sum_{d \in V} \frac{1}{2} {}^1T_{c,k} Y_{a,\gamma}^{1,*} Y_{i,\gamma}^{2,*} Z_{\gamma,\zeta}^* Y_{b,\zeta}^{3,*} {}^2D_{a,i,b,j} {}^2T_{b,j,d,i} V_{a,c,k,d} \quad (11687)$$

Factorized expression

$$\tau_{\gamma,\delta,w}^0 = \sum_{a \in V} {}^2D_{a,w}^3 Y_{a,\gamma}^3 Y_{a,\delta}^{3,*} \quad (3r_D r_T^2 N_v) \quad (11688)$$

$$\tau_{\gamma,\delta,w}^1 = \sum_{i \in O} {}^2D_{i,w}^2 Y_{i,\gamma}^2 Y_{i,\delta}^{2,*} \quad (3r_D r_T^2 N_o) \quad (11689)$$

$$\tau_{\alpha,i}^2 = \sum_{a \in V} {}^1T_{a,i} W_{a,\alpha}^2 \quad (2r_V N_o N_v) \quad (11690)$$

$$\tau_{\alpha,\beta}^3 = \sum_{i \in O} W_{i,\beta}^3 \tau_{\alpha,i}^2 \quad (2r_V^2 N_o) \quad (11691)$$

$$\tau_{\alpha,a}^4 = \sum_{\beta \in B} X_{\alpha,\beta} W_{a,\beta}^4 \tau_{\alpha,\beta}^3 \quad (3r_V^2 N_v) \quad (11692)$$

$$\tau_{a,b}^5 = \sum_{\alpha \in B} W_{a,\alpha}^1 \tau_{\alpha,b}^4 \quad (2r_V N_v^2) \quad (11693)$$

$$\tau_{\gamma,a}^6 = \sum_{b \in V} Y_{b,\gamma}^1 \tau_{a,b}^5 \quad (2r_T N_v^2) \quad (11694)$$

$$\tau_{\gamma,\delta,w}^7 = \sum_{a \in V} {}^2D_{a,w}^1 Y_{a,w}^{1,*} \tau_{\gamma,a}^6 \quad (3r_D r_T^2 N_v) \quad (11695)$$

$$\tau_{\gamma,\delta,w}^8 = \sum_{\epsilon \in A} Z_{\epsilon,\delta}^* \tau_{\gamma,\epsilon,w}^1 \tau_{\gamma,\epsilon,w}^7 \quad (3r_D r_T^3) \quad (11696)$$

$$\tau_{\gamma,\delta,w}^9 = \sum_{\epsilon \in A} Z_{\epsilon,\gamma} \tau_{\epsilon,\delta,w}^8 \quad (2r_D r_T^3) \quad (11697)$$

$${}^2R_{i,\gamma}^4 \leftarrow - \sum_{\delta \in A} \sum_{w \in D} \frac{1}{2} {}^2D_{i,w}^4 Y_{i,\delta}^4 \tau_{\delta,\gamma,w}^5 \tau_{\delta,\gamma,w}^9 \quad (4r_D r_T^2 N_o) \quad (11710)$$

$${}^2R_{i,\gamma}^4 \leftarrow - \sum_{\delta \in A} \sum_{w \in D} \frac{1}{2} {}^2D_{i,w}^4 Y_{i,\delta}^4 \tau_{\delta,\gamma,w}^0 \tau_{\delta,\gamma,w}^9 \quad (4r_D r_T^2 N_o) \quad \text{Raw expression} \quad (11698)$$

$${}^2R_{j,\zeta}^4 \leftarrow - \sum_{\gamma \in A} \sum_{i \in O} \sum_{k \in O} \sum_{a \in V} \sum_{b \in V} \sum_{c \in V} \sum_{d \in V} \frac{1}{2} {}^1T_{c,k} Y_{a,\gamma}^{1,*} Y_{i,\gamma}^{2,*} Z_{\gamma,\zeta}^* Y_{b,\zeta}^{3,*} {}^2D_{a,i,b,j} {}^2T_{d,j,a,i} V_{b,c,k,d} \quad (11711)$$

Raw expression

$${}^2R_{j,\zeta}^4 \leftarrow - \sum_{\gamma \in A} \sum_{i \in O} \sum_{k \in O} \sum_{a \in V} \sum_{b \in V} \sum_{c \in V} \sum_{d \in V} \frac{1}{2} {}^1T_{c,k} Y_{a,\gamma}^{1,*} Y_{i,\gamma}^{2,*} Z_{\gamma,\zeta}^* Y_{b,\zeta}^{3,*} {}^2D_{a,i,b,j} {}^2T_{d,i,b,j} V_{a,c,k,d} \quad (11699)$$

Factorized expression

$$\tau_{\alpha,i}^0 = \sum_{a \in V} {}^1T_{a,i} W_{a,\alpha}^2 \quad (2r_V N_o N_v) \quad (11712)$$

Factorized expression

$$\tau_{\alpha,i}^0 = \sum_{a \in V} {}^1T_{a,i} W_{a,\alpha}^2 \quad (2r_V N_o N_v) \quad (11700)$$

$$\tau_{\alpha,\beta}^1 = \sum_{i \in O} W_{i,\beta}^3 \tau_{\alpha,i}^0 \quad (2r_V^2 N_o) \quad (11713)$$

$$\tau_{\alpha,\beta}^1 = \sum_{i \in O} W_{i,\beta}^3 \tau_{\alpha,i}^0 \quad (2r_V^2 N_o) \quad (11701)$$

$$\tau_{\alpha,a}^2 = \sum_{\beta \in B} X_{\alpha,\beta} W_{a,\beta}^4 \tau_{\alpha,\beta}^1 \quad (3r_V^2 N_v) \quad (11714)$$

$$\tau_{\alpha,a}^2 = \sum_{\beta \in B} X_{\alpha,\beta} W_{a,\beta}^4 \tau_{\alpha,\beta}^1 \quad (3r_V^2 N_v) \quad (11702)$$

$$\tau_{a,b}^3 = \sum_{\alpha \in B} W_{a,\alpha}^1 \tau_{\alpha,b}^2 \quad (2r_V N_v^2) \quad (11715)$$

$$\tau_{a,b}^3 = \sum_{\alpha \in B} W_{a,\alpha}^1 \tau_{\alpha,b}^2 \quad (2r_V N_v^2) \quad (11703)$$

$$\tau_{\gamma,a}^4 = \sum_{b \in V} Y_{b,\gamma}^1 \tau_{a,b}^3 \quad (2r_T N_v^2) \quad (11716)$$

$$\tau_{\gamma,a}^4 = \sum_{b \in V} Y_{b,\gamma}^1 \tau_{a,b}^3 \quad (2r_T N_v^2) \quad (11704)$$

$$\tau_{\gamma,\delta,w}^5 = \sum_{a \in V} {}^2D_{a,w}^3 Y_{a,\delta}^{3,*} \tau_{\gamma,a}^4 \quad (3r_D r_T^2 N_v) \quad (11717)$$

$$\tau_{\gamma,\delta,w}^5 = \sum_{a \in V} {}^2D_{a,w}^3 Y_{a,\delta}^{3,*} \tau_{\gamma,a}^4 \quad (3r_D r_T^2 N_v) \quad (11705)$$

$$\tau_{\gamma,\delta,w}^6 = \sum_{a \in V} {}^2D_{a,w}^1 Y_{a,\gamma}^3 Y_{a,\delta}^{1,*} \quad (3r_D r_T^2 N_v) \quad (11718)$$

$$\tau_{\gamma,\delta,w}^6 = \sum_{a \in V} {}^2D_{a,w}^1 Y_{a,\gamma}^1 Y_{a,\delta}^{1,*} \quad (3r_D r_T^2 N_v) \quad (11706)$$

$$\tau_{\gamma,\delta,w}^7 = \sum_{i \in O} {}^2D_{i,w}^2 Y_{i,\gamma}^4 Y_{i,\delta}^{2,*} \quad (3r_D r_T^2 N_o) \quad (11719)$$

$$\tau_{\gamma,\delta,w}^7 = \sum_{i \in O} {}^2D_{i,w}^2 Y_{i,\gamma}^2 Y_{i,\delta}^{2,*} \quad (3r_D r_T^2 N_o) \quad (11707)$$

$$\tau_{\gamma,\delta,w}^8 = \sum_{\epsilon \in A} Z_{\epsilon,\delta}^* \tau_{\gamma,\epsilon,w}^6 \tau_{\gamma,\epsilon,w}^7 \quad (3r_D r_T^3) \quad (11720)$$

$$\tau_{\gamma,\delta,w}^8 = \sum_{\epsilon \in A} Z_{\epsilon,\delta}^* \tau_{\gamma,\epsilon,w}^6 \tau_{\gamma,\epsilon,w}^7 \quad (3r_D r_T^3) \quad (11708)$$

$$\tau_{\gamma,\delta,w}^9 = \sum_{\epsilon \in A} Z_{\gamma,\epsilon} \tau_{\epsilon,\delta,w}^8 \quad (2r_D r_T^3) \quad (11721)$$

$$\tau_{\gamma,\delta,w}^9 = \sum_{\epsilon \in A} Z_{\epsilon,\gamma} \tau_{\epsilon,\delta,w}^8 \quad (2r_D r_T^3) \quad (11709)$$

$${}^2R_{i,\gamma}^4 \leftarrow - \sum_{\delta \in A} \sum_{w \in D} \frac{1}{2} {}^2D_{i,w}^4 Y_{i,\delta}^2 \tau_{\delta,\gamma,w}^5 \tau_{\delta,\gamma,w}^9 \quad (4r_D r_T^2 N_o) \quad (11722)$$

Raw expression

$${}^2R^4_{j,\zeta} \leftarrow \sum_{\gamma \in A} \sum_{i \in O} \sum_{k \in O} \sum_{l \in O} \sum_{a \in V} \sum_{b \in V} \sum_{c \in V} \frac{1}{2} {}^1T_{a,k} {}^Y{}^{1,*}_{a,\gamma} {}^Y{}^{2,*}_{i,\gamma} {}^Z{}^*_{\gamma,\zeta} {}^Y{}^{3,*}_{b,\zeta} {}^2D^{a,i,b,j} {}^2T_{b,j,c,l} {}^V_{l,i,k,c} \quad (11723)$$

Factorized expression

$$\tau^0_{\gamma,\delta,w} = \sum_{a \in V} {}^2D^3_{a,w} {}^Y{}^1_{a,\gamma} {}^Y{}^{3,*}_{a,\delta} \quad (3r_D r_T^2 N_v) \quad (11724)$$

$$\tau^1_{\gamma,w,i} = \sum_{a \in V} {}^2D^1_{a,w} {}^1T_{a,i} {}^Y{}^{1,*}_{a,\gamma} \quad (3r_D r_T N_o N_v) \quad (11725)$$

$$\tau^2_{\gamma,\alpha,w} = \sum_{i \in O} W^1_{i,\alpha} \tau^1_{\gamma,w,i} \quad (2r_D r_T r_V N_o) \quad (11726)$$

$$\tau^3_{\gamma,\alpha,w} = \sum_{i \in O} {}^2D^2_{i,w} W^2_{i,\alpha} {}^Y{}^{2,*}_{i,\gamma} \quad (3r_D r_T r_V N_o) \quad (11727)$$

$$\tau^4_{\gamma,\alpha} = \sum_{a \in V} W^4_{a,\alpha} {}^Y{}^3_{a,\gamma} \quad (2r_T r_V N_v) \quad (11728)$$

$$\tau^5_{\gamma,\alpha} = \sum_{i \in O} W^3_{i,\alpha} {}^Y{}^4_{i,\gamma} \quad (2r_T r_V N_o) \quad (11729)$$

$$\tau^6_{\gamma,\alpha} = \sum_{\beta \in B} X_{\alpha,\beta} \tau^4_{\gamma,\beta} \tau^5_{\gamma,\beta} \quad (3r_T r_V^2) \quad (11730)$$

$$\tau^7_{\gamma,\alpha} = \sum_{\delta \in A} Z_{\gamma,\delta} \tau^6_{\delta,\alpha} \quad (2r_T^2 r_V) \quad (11731)$$

$$\tau^8_{\gamma,\delta,w} = \sum_{\alpha \in B} \tau^7_{\gamma,\alpha} \tau^2_{\delta,\alpha,w} \tau^3_{\delta,\alpha,w} \quad (3r_D r_T^2 r_V) \quad (11732)$$

$$\tau^9_{\gamma,\delta,w} = \sum_{\epsilon \in A} Z^*_{\epsilon,\delta} \tau^8_{\gamma,\epsilon,w} \quad (2r_D r_T^3) \quad (11733)$$

$${}^2R^4_{i,\gamma} \leftarrow - \sum_{\delta \in A} \sum_{w \in D} {}^2D^4_{i,w} {}^Y{}^2_{i,\delta} \tau^0_{\delta,\gamma,w} \tau^9_{\delta,\gamma,w} \quad (4r_D r_T^2 N_o) \quad (11734)$$

Raw expression

$${}^2R^4_{j,\zeta} \leftarrow \sum_{\gamma \in A} \sum_{i \in O} \sum_{k \in O} \sum_{l \in O} \sum_{a \in V} \sum_{b \in V} \sum_{c \in V} \frac{1}{2} {}^1T_{a,k} {}^Y{}^{1,*}_{a,\gamma} {}^Y{}^{2,*}_{i,\gamma} {}^Z{}^*_{\gamma,\zeta} {}^Y{}^{3,*}_{b,\zeta} {}^2D^{a,i,b,j} {}^2T_{b,l,c,i} {}^V_{k,c,l,j} \quad (11735)$$

Factorized expression

$$\tau^0_{\gamma,\delta,w} = \sum_{a \in V} {}^2D^3_{a,w} {}^Y{}^3_{a,\gamma} {}^Y{}^{3,*}_{a,\delta} \quad (3r_D r_T^2 N_v) \quad (11736)$$

$$\tau^1_{\gamma,w,i} = \sum_{a \in V} {}^2D^1_{a,w} {}^1T_{a,i} {}^Y{}^{1,*}_{a,\gamma} \quad (3r_D r_T N_o N_v) \quad (11737)$$

$$\tau^2_{\gamma,\alpha,w} = \sum_{i \in O} W^1_{i,\alpha} \tau^1_{\gamma,w,i} \quad (2r_D r_T r_V N_o) \quad (11738)$$

$$\tau^3_{\gamma,\alpha,w} = \sum_{i \in O} {}^2D^2_{i,w} W^2_{i,\alpha} {}^Y{}^{2,*}_{i,\gamma} \quad (3r_D r_T r_V N_o) \quad (11739)$$

$$\tau^4_{\gamma,\alpha} = \sum_{a \in V} W^4_{a,\alpha} {}^Y{}^1_{a,\gamma} \quad (2r_T r_V N_v) \quad (11740)$$

$$\tau^5_{\gamma,\alpha} = \sum_{i \in O} W^3_{i,\alpha} {}^Y{}^2_{i,\gamma} \quad (2r_T r_V N_o) \quad (11741)$$

$$\tau^6_{\gamma,\alpha} = \sum_{\beta \in B} X_{\alpha,\beta} \tau^4_{\gamma,\beta} \tau^5_{\gamma,\beta} \quad (3r_T r_V^2) \quad (11742)$$

$$\tau^7_{\gamma,\alpha} = \sum_{\delta \in A} Z_{\delta,\gamma} \tau^6_{\delta,\alpha} \quad (2r_T^2 r_V) \quad (11743)$$

$$\tau^8_{\gamma,\delta,w} = \sum_{\alpha \in B} \tau^7_{\gamma,\alpha} \tau^2_{\delta,\alpha,w} \tau^3_{\delta,\alpha,w} \quad (3r_D r_T^2 r_V) \quad (11744)$$

$$\tau^9_{\gamma,\delta,w} = \sum_{\epsilon \in A} Z^*_{\epsilon,\delta} \tau^8_{\gamma,\epsilon,w} \quad (2r_D r_T^3) \quad (11745)$$

$${}^2R^4_{i,\gamma} \leftarrow - \sum_{\delta \in A} \sum_{w \in D} {}^2D^4_{i,w} {}^Y{}^4_{i,\delta} \tau^0_{\delta,\gamma,w} \tau^9_{\delta,\gamma,w} \quad (4r_D r_T^2 N_o) \quad (11746)$$

Raw expression

$${}^2R^4_{j,\zeta} \leftarrow \sum_{\gamma \in A} \sum_{i \in O} \sum_{k \in O} \sum_{l \in O} \sum_{a \in V} \sum_{b \in V} \sum_{c \in V} \frac{1}{2} {}^1T_{a,k} Y^{1,*}_{a,\gamma} Y^{2,*}_{i,\gamma} Z^*_{\gamma,\zeta} Y^{3,*}_{b,\zeta} {}^2D^{a,i,b,j} {}^2T_{b,l,c,j} V_{k,i,l,c} \quad (11747)$$

Factorized expression

$$\tau^0_{\gamma,\alpha} = \sum_{a \in V} W^2_{a,\alpha} Y^3_{a,\gamma} \quad (2r_T r_V N_v) \quad (11748)$$

$$\tau^1_{\gamma,\alpha} = \sum_{i \in O} W^1_{i,\alpha} Y^4_{i,\gamma} \quad (2r_T r_V N_o) \quad (11749)$$

$$\tau^2_{\gamma,\alpha} = \sum_{\beta \in B} X_{\beta,\alpha} \tau^0_{\gamma,\beta} \tau^1_{\gamma,\beta} \quad (3r_T r_V^2) \quad (11750)$$

$$\tau^3_{\gamma,\alpha} = \sum_{\delta \in A} Z_{\gamma,\delta} \tau^2_{\delta,\alpha} \quad (2r_T^2 r_V) \quad (11751)$$

$$\tau^4_{\gamma,\delta,w} = \sum_{a \in V} {}^2D^1_{a,w} Y^1_{a,\gamma} Y^{1,*}_{a,\delta} \quad (3r_D r_T^2 N_v) \quad (11752)$$

$$\tau^5_{\gamma,\delta,w} = \sum_{i \in O} {}^2D^2_{i,w} Y^2_{i,\gamma} Y^{2,*}_{i,\delta} \quad (3r_D r_T^2 N_o) \quad (11753)$$

$$\tau^6_{\gamma,\delta,w} = \sum_{\epsilon \in A} Z^*_{\epsilon,\delta} \tau^4_{\gamma,\epsilon,w} \tau^5_{\gamma,\epsilon,w} \quad (3r_D r_T^3) \quad (11754)$$

$$\tau^7_{\gamma,\alpha,w} = \sum_{\delta \in A} \tau^3_{\delta,\alpha} \tau^6_{\delta,\gamma,w} \quad (2r_D r_T^2 r_V) \quad (11755)$$

$$\tau^8_{\gamma,w,i} = \sum_{a \in V} {}^2D^3_{a,w} {}^1T_{a,i} Y^{3,*}_{a,\gamma} \quad (3r_D r_T N_o N_v) \quad (11756)$$

$$\tau^9_{\gamma,\alpha,w} = \sum_{i \in O} W^3_{i,\alpha} \tau^8_{\gamma,w,i} \quad (2r_D r_T r_V N_o) \quad (11757)$$

$$\tau^{10}_{\gamma,w,i} = \sum_{\alpha \in B} W^4_{i,\alpha} \tau^7_{\gamma,\alpha,w} \tau^9_{\gamma,\alpha,w} \quad (3r_D r_T r_V N_o) \quad (11758)$$

$${}^2R^4_{i,\gamma} \leftarrow - \sum_{w \in D} {}^2D^4_{i,w} \tau^{10}_{\gamma,w,i} \quad (2r_D r_T N_o) \quad (11759)$$

Raw expression

$${}^2R^4_{j,\zeta} \leftarrow \sum_{\gamma \in A} \sum_{i \in O} \sum_{k \in O} \sum_{l \in O} \sum_{a \in V} \sum_{b \in V} \sum_{c \in V} \frac{1}{2} {}^1T_{a,k} Y^{1,*}_{a,\gamma} Y^{2,*}_{i,\gamma} Z^*_{\gamma,\zeta} Y^{3,*}_{b,\zeta} {}^2D^{a,i,b,j} {}^2T_{c,i,b,l} V_{k,c,l,j} \quad (11760)$$

Factorized expression

$$\tau^0_{\gamma,\delta,w} = \sum_{a \in V} {}^2D^1_{a,w} Y^3_{a,\gamma} Y^{1,*}_{a,\delta} \quad (3r_D r_T^2 N_v) \quad (11761)$$

$$\tau^1_{\gamma,\delta,w} = \sum_{i \in O} {}^2D^2_{i,w} Y^4_{i,\gamma} Y^{2,*}_{i,\delta} \quad (3r_D r_T^2 N_o) \quad (11762)$$

$$\tau^2_{\gamma,\delta,w} = \sum_{\epsilon \in A} Z^*_{\epsilon,\delta} \tau^0_{\gamma,\epsilon,w} \tau^1_{\gamma,\epsilon,w} \quad (3r_D r_T^3) \quad (11763)$$

$$\tau^3_{\gamma,\alpha} = \sum_{a \in V} W^2_{a,\alpha} Y^1_{a,\gamma} \quad (2r_T r_V N_v) \quad (11764)$$

$$\tau^4_{\gamma,\alpha} = \sum_{i \in O} W^1_{i,\alpha} Y^2_{i,\gamma} \quad (2r_T r_V N_o) \quad (11765)$$

$$\tau^5_{\gamma,\alpha} = \sum_{\beta \in B} X_{\beta,\alpha} \tau^3_{\gamma,\beta} \tau^4_{\gamma,\beta} \quad (3r_T r_V^2) \quad (11766)$$

$$\tau^6_{\gamma,\alpha} = \sum_{\delta \in A} Z_{\delta,\gamma} \tau^5_{\delta,\alpha} \quad (2r_T^2 r_V) \quad (11767)$$

$$\tau^7_{\gamma,\alpha,w} = \sum_{\delta \in A} \tau^6_{\delta,\alpha} \tau^2_{\delta,\gamma,w} \quad (2r_D r_T^2 r_V) \quad (11768)$$

$$\tau^8_{\gamma,w,i} = \sum_{a \in V} {}^2D^3_{a,w} {}^1T_{a,i} Y^{3,*}_{a,\gamma} \quad (3r_D r_T N_o N_v) \quad (11769)$$

$$\tau^9_{\gamma,\alpha,w} = \sum_{i \in O} W^3_{i,\alpha} \tau^8_{\gamma,w,i} \quad (2r_D r_T r_V N_o) \quad (11770)$$

$$\tau^{10}_{\gamma,w,i} = \sum_{\alpha \in B} W^4_{i,\alpha} \tau^7_{\gamma,\alpha,w} \tau^9_{\gamma,\alpha,w} \quad (3r_D r_T r_V N_o) \quad (11771)$$

$${}^2R^4_{i,\gamma} \leftarrow - \sum_{w \in D} {}^2D^4_{i,w} \tau^{10}_{\gamma,w,i} \quad (2r_D r_T N_o) \quad (11772)$$

Raw expression



$${}^2R^4_{j,\zeta} \leftarrow \sum_{\gamma \in A} \sum_{i \in O} \sum_{k \in O} \sum_{l \in O} \sum_{a \in V} \sum_{b \in V} \sum_{c \in V} \frac{1}{2} {}^1T_{a,k} Y^{1,*}_{a,\gamma} Y^{2,*}_{i,\gamma} Z^*_{\gamma,\zeta} Y^{3,*}_{b,\zeta} {}^2D^{a,i,b,j} {}^2T_{c,j,b,l} V_{k,i,l,c} \quad (11773)$$

Factorized expression

$$\tau^0_{\gamma,\delta,w} = \sum_{a \in V} {}^2D^3_{a,w} Y^3_{a,\gamma} Y^{3,*}_{a,\delta} \quad (3r_D r_T^2 N_v) \quad (11774)$$

$$\tau^1_{\gamma,\delta,w} = \sum_{a \in V} {}^2D^1_{a,w} Y^1_{a,\gamma} Y^{1,*}_{a,\delta} \quad (3r_D r_T^2 N_v) \quad (11775)$$

$$\tau^2_{\gamma,\delta,w} = \sum_{i \in O} {}^2D^2_{i,w} Y^2_{i,\gamma} Y^{2,*}_{i,\delta} \quad (3r_D r_T^2 N_o) \quad (11776)$$

$$\tau^3_{\gamma,\delta,w} = \sum_{\epsilon \in A} Z^*_{\epsilon,\delta} \tau^1_{\gamma,\epsilon,w} \tau^2_{\gamma,\epsilon,w} \quad (3r_D r_T^3) \quad (11777)$$

$$\tau^4_{\gamma,\delta,w} = \sum_{\epsilon \in A} Z_{\epsilon,\gamma} \tau^3_{\epsilon,\delta,w} \quad (2r_D r_T^3) \quad (11778)$$

$$\tau^5_{\alpha,i} = \sum_{a \in V} {}^1T_{a,i} W^2_{a,\alpha} \quad (2r_V N_o N_v) \quad (11779)$$

$$\tau^6_{\alpha} = \sum_{i \in O} W^1_{i,\alpha} \tau^5_{\alpha,i} \quad (2r_V N_o) \quad (11780)$$

$$\tau^7_{\alpha} = \sum_{\beta \in B} \tau^6_{\beta} X_{\beta,\alpha} \quad (2r_V^2) \quad (11781)$$

$$\tau^8_{i,j} = \sum_{\alpha \in B} \tau^7_{\alpha} W^3_{i,\alpha} W^4_{j,\alpha} \quad (3r_V N_o^2) \quad (11782)$$

$$\tau^9_{\gamma,i} = \sum_{j \in O} Y^4_{j,\gamma} \tau^8_{j,i} \quad (2r_T N_o^2) \quad (11783)$$

$${}^2R^4_{i,\gamma} \leftarrow - \sum_{\delta \in A} \sum_{w \in D} {}^2D^4_{i,w} \tau^9_{\delta,i} \tau^0_{\delta,\gamma,w} \tau^4_{\delta,\gamma,w} \quad (4r_D r_T^2 N_o) \quad (11784)$$

Raw expression

$${}^2R^4_{j,\zeta} \leftarrow \sum_{\gamma \in A} \sum_{i \in O} \sum_{k \in O} \sum_{l \in O} \sum_{a \in V} \sum_{b \in V} \sum_{c \in V} \frac{1}{2} {}^1T_{a,k} Y^{1,*}_{a,\gamma} Y^{2,*}_{i,\gamma} Z^*_{\gamma,\zeta} Y^{3,*}_{b,\zeta} {}^2D^{a,i,b,j} {}^2T_{c,l,b,j} V_{l,i,k,c} \quad (11785)$$

Factorized expression

$$\tau^0_{\gamma,\delta,w} = \sum_{a \in V} {}^2D^3_{a,w} Y^1_{a,\gamma} Y^{3,*}_{a,\delta} \quad (3r_D r_T^2 N_v) \quad (11786)$$

$$\tau^1_{\gamma,\delta,w} = \sum_{a \in V} {}^2D^1_{a,w} Y^3_{a,\gamma} Y^{1,*}_{a,\delta} \quad (3r_D r_T^2 N_v) \quad (11787)$$

$$\tau^2_{\gamma,\delta,w} = \sum_{i \in O} {}^2D^2_{i,w} Y^4_{i,\gamma} Y^{2,*}_{i,\delta} \quad (3r_D r_T^2 N_o) \quad (11788)$$

$$\tau^3_{\gamma,\delta,w} = \sum_{\epsilon \in A} Z^*_{\epsilon,\delta} \tau^1_{\gamma,\epsilon,w} \tau^2_{\gamma,\epsilon,w} \quad (3r_D r_T^3) \quad (11789)$$

$$\tau^4_{\gamma,\delta,w} = \sum_{\epsilon \in A} Z_{\gamma,\epsilon} \tau^3_{\epsilon,\delta,w} \quad (2r_D r_T^3) \quad (11790)$$

$$\tau^5_{\alpha,i} = \sum_{a \in V} {}^1T_{a,i} W^2_{a,\alpha} \quad (2r_V N_o N_v) \quad (11791)$$

$$\tau^6_{\alpha} = \sum_{i \in O} W^1_{i,\alpha} \tau^5_{\alpha,i} \quad (2r_V N_o) \quad (11792)$$

$$\tau^7_{\alpha} = \sum_{\beta \in B} \tau^6_{\beta} X_{\beta,\alpha} \quad (2r_V^2) \quad (11793)$$

$$\tau^8_{i,j} = \sum_{\alpha \in B} \tau^7_{\alpha} W^3_{i,\alpha} W^4_{j,\alpha} \quad (3r_V N_o^2) \quad (11794)$$

$$\tau^9_{\gamma,i} = \sum_{j \in O} Y^2_{j,\gamma} \tau^8_{j,i} \quad (2r_T N_o^2) \quad (11795)$$

$${}^2R^4_{i,\gamma} \leftarrow - \sum_{\delta \in A} \sum_{w \in D} {}^2D^4_{i,w} \tau^9_{\delta,i} \tau^0_{\delta,\gamma,w} \tau^4_{\delta,\gamma,w} \quad (4r_D r_T^2 N_o) \quad (11796)$$

Raw expression

$${}^2R^4_{j,\zeta} \leftarrow \sum_{\gamma \in A} \sum_{i \in O} \sum_{k \in O} \sum_{l \in O} \sum_{a \in V} \sum_{b \in V} \sum_{c \in V} \frac{1}{2} {}^1T_{b,k} Y^{1,*}_{a,\gamma} Y^{2,*}_{i,\gamma} Z^*_{\gamma,\zeta} Y^{3,*}_{b,\zeta} {}^2D^{a,i,b,j} {}^2T_{a,i,c,l} V_{k,c,l,j} \quad (11797)$$

Factorized expression

$$\tau^0_{\gamma,\delta,w} = \sum_{a \in V} {}^2D^3_{a,w} Y^3_{a,\gamma} Y^{3,*}_{a,\delta} \quad (3r_D r_T^2 N_v) \quad (11798)$$

$$\tau^1_{\gamma,\delta,w} = \sum_{a \in V} {}^2D^1_{a,w} Y^3_{a,\gamma} Y^{1,*}_{a,\delta} \quad (3r_D r_T^2 N_v) \quad (11811)$$

$$\tau^1_{\gamma,\delta,w} = \sum_{a \in V} {}^2D^1_{a,w} Y^1_{a,\gamma} Y^{1,*}_{a,\delta} \quad (3r_D r_T^2 N_v) \quad (11799)$$

$$\tau^2_{\alpha,i} = \sum_{a \in V} {}^1T_{a,i} W^4_{a,\alpha} \quad (2r_V N_o N_v) \quad (11812)$$

$$\tau^2_{\alpha,i} = \sum_{a \in V} {}^1T_{a,i} W^4_{a,\alpha} \quad (2r_V N_o N_v) \quad (11800)$$

$$\tau^3_{\alpha} = \sum_{i \in O} W^3_{i,\alpha} \tau^2_{\alpha,i} \quad (2r_V N_o) \quad (11813)$$

$$\tau^3_{\alpha} = \sum_{i \in O} W^3_{i,\alpha} \tau^2_{\alpha,i} \quad (2r_V N_o) \quad (11801)$$

$$\tau^4_{\alpha} = \sum_{\beta \in B} \tau^3_{\beta} X_{\alpha,\beta} \quad (2r_V^2) \quad (11814)$$

$$\tau^4_{\alpha} = \sum_{\beta \in B} \tau^3_{\beta} X_{\alpha,\beta} \quad (2r_V^2) \quad (11802)$$

$$\tau^5_{i,j} = \sum_{\alpha \in B} \tau^4_{\alpha} W^1_{i,\alpha} W^2_{j,\alpha} \quad (3r_V N_o^2) \quad (11815)$$

$$\tau^5_{i,j} = \sum_{\alpha \in B} \tau^4_{\alpha} W^1_{i,\alpha} W^2_{j,\alpha} \quad (3r_V N_o^2) \quad (11803)$$

$$\tau^6_{\gamma,i} = \sum_{j \in O} Y^4_{j,\gamma} \tau^5_{j,i} \quad (2r_T N_o^2) \quad (11816)$$

$$\tau^6_{\gamma,i} = \sum_{j \in O} Y^2_{j,\gamma} \tau^5_{j,i} \quad (2r_T N_o^2) \quad (11804)$$

$$\tau^7_{\gamma,\delta,w} = \sum_{i \in O} {}^2D^2_{i,w} Y^{2,*}_{i,\delta} \tau^6_{\gamma,i} \quad (3r_D r_T^2 N_o) \quad (11817)$$

$$\tau^7_{\gamma,\delta,w} = \sum_{i \in O} {}^2D^2_{i,w} Y^{2,*}_{i,\delta} \tau^6_{\gamma,i} \quad (3r_D r_T^2 N_o) \quad (11805)$$

$$\tau^8_{\gamma,\delta,w} = \sum_{\epsilon \in A} Z^*_{\epsilon,\delta} \tau^1_{\gamma,\epsilon,w} \tau^7_{\gamma,\epsilon,w} \quad (3r_D r_T^3) \quad (11818)$$

$$\tau^8_{\gamma,\delta,w} = \sum_{\epsilon \in A} Z^*_{\epsilon,\delta} \tau^1_{\gamma,\epsilon,w} \tau^7_{\gamma,\epsilon,w} \quad (3r_D r_T^3) \quad (11806)$$

$$\tau^9_{\gamma,\delta,w} = \sum_{\epsilon \in A} Z_{\gamma,\epsilon} \tau^8_{\epsilon,\delta,w} \quad (2r_D r_T^3) \quad (11819)$$

$$\tau^9_{\gamma,\delta,w} = \sum_{\epsilon \in A} Z_{\epsilon,\gamma} \tau^8_{\epsilon,\delta,w} \quad (2r_D r_T^3) \quad (11807)$$

$${}^2R^4_{i,\gamma} \leftarrow - \sum_{\delta \in A} \sum_{w \in D} {}^2D^4_{i,w} Y^2_{i,\delta} \tau^0_{\delta,\gamma,w} \tau^9_{\delta,\gamma,w} \quad (4r_D r_T^2 N_o) \quad (11820)$$

$${}^2R^4_{i,\gamma} \leftarrow - \sum_{\gamma \in A} \sum_{\delta \in A} \sum_{w \in D} {}^2D^4_{i,w} Y^4_{i,\delta} \tau^0_{\delta,\gamma,w} \tau^9_{\delta,\gamma,w} \quad (4r_D r_T^2 N_o) \quad (11808)$$

Raw expression

$${}^2R^4_{j,\zeta} \leftarrow \sum_{\gamma \in A} \sum_{i \in O} \sum_{k \in O} \sum_{l \in O} \sum_{a \in V} \sum_{b \in V} \sum_{c \in V} \frac{1}{2} {}^1T_{b,k} Y^{1,*}_{a,\gamma} Y^{2,*}_{i,\gamma} Z^*_{\gamma,\zeta} Y^{3,*}_{b,\zeta} {}^2D^{a,i,b,j} {}^2T_{a,l,c,j} V_{l,c,k,j} \quad (11809)$$

Factorized expression

$$\tau^0_{\gamma,\delta,w} = \sum_{a \in V} {}^2D^3_{a,w} Y^1_{a,\gamma} Y^{3,*}_{a,\delta} \quad (3r_D r_T^2 N_v) \quad (11810)$$

Raw expression

$${}^2R^4_{j,\zeta} \leftarrow \sum_{\gamma \in A} \sum_{i \in O} \sum_{k \in O} \sum_{l \in O} \sum_{a \in V} \sum_{b \in V} \sum_{c \in V} \frac{1}{2} {}^1T_{b,k} Y^{1,*}_{a,\gamma} Y^{2,*}_{i,\gamma} Z^*_{\gamma,\zeta} Y^{3,*}_{b,\zeta} {}^2D^{a,i,b,j} {}^2T_{a,l,c,j} V_{l,i,k,c} \quad (11821)$$

Factorized expression

$$\tau^0_{\gamma,\delta,w} = \sum_{a \in V} {}^2D^3_{a,w} Y^1_{a,\gamma} Y^{3,*}_{a,\delta} \quad (3r_D r_T^2 N_v) \quad (11822)$$

$$\tau^1_{\gamma,w,i} = \sum_{a \in V} {}^2D^1_{a,w} {}^1T_{a,i} Y^{1,*}_{a,\gamma} \quad (3r_D r_T N_o N_v) \quad (11823)$$

$$\tau_{\gamma,w,i,j}^2 = \sum_{\delta \in A} {}^2D_{i,w}^2 Y_{i,\delta}^{2,*} Z_{\delta,\gamma}^* \tau_{\delta,w,j}^1 \quad (4r_D r_T^2 N_o^2) \quad (11824)$$

$$\tau_{\gamma,w,i,j}^2 = \sum_{\delta \in A} {}^2D_{i,w}^2 Y_{i,\delta}^{2,*} Z_{\delta,\gamma}^* \tau_{\delta,w,j}^1 \quad (4r_D r_T^2 N_o^2) \quad (11837)$$

$$\tau_{\gamma,\alpha,w,i}^3 = \sum_{j \in O} W_{j,\alpha}^1 \tau_{\gamma,w,i,j}^2 \quad (2r_D r_T r_V N_o^2) \quad (11825)$$

$$\tau_{\gamma,\alpha,w,i}^3 = \sum_{j \in O} W_{j,\alpha}^1 \tau_{\gamma,w,i,j}^2 \quad (2r_D r_T r_V N_o^2) \quad (11838)$$

$$\tau_{\gamma,\alpha}^4 = \sum_{a \in V} W_{a,\alpha}^2 Y_{a,\gamma}^3 \quad (2r_T r_V N_v) \quad (11826)$$

$$\tau_{\gamma,\alpha}^4 = \sum_{a \in V} W_{a,\alpha}^2 Y_{a,\gamma}^1 \quad (2r_T r_V N_v) \quad (11839)$$

$$\tau_{\gamma,\alpha,i}^5 = \sum_{\delta \in A} Z_{\gamma,\delta} Y_{i,\delta}^4 \tau_{\delta,\alpha}^4 \quad (3r_T^2 r_V N_o) \quad (11827)$$

$$\tau_{\gamma,\alpha,i}^5 = \sum_{\delta \in A} Y_{i,\delta}^2 Z_{\delta,\gamma} \tau_{\delta,\alpha}^4 \quad (3r_T^2 r_V N_o) \quad (11840)$$

$$\tau_{\gamma,\delta,\alpha,w}^6 = \sum_{i \in O} \tau_{\gamma,\alpha,i}^5 \tau_{\delta,\alpha,w,i}^3 \quad (2r_D r_T^2 r_V N_o) \quad (11828)$$

$$\tau_{\gamma,\delta,\alpha,w}^6 = \sum_{i \in O} \tau_{\gamma,\alpha,i}^5 \tau_{\delta,\alpha,w,i}^3 \quad (2r_D r_T^2 r_V N_o) \quad (11841)$$

$$\tau_{\alpha,i,j}^7 = \sum_{\beta \in B} X_{\alpha,\beta} W_{i,\beta}^3 W_{j,\beta}^4 \quad (3r_V^2 N_o^2) \quad (11829)$$

$$\tau_{\alpha,i,j}^7 = \sum_{\beta \in B} X_{\alpha,\beta} W_{i,\beta}^3 W_{j,\beta}^4 \quad (3r_V^2 N_o^2) \quad (11842)$$

$$\tau_{\gamma,\alpha,i}^8 = \sum_{j \in O} Y_{j,\gamma}^2 \tau_{\alpha,j,i}^7 \quad (2r_T r_V N_o^2) \quad (11830)$$

$$\tau_{\gamma,\alpha,i}^8 = \sum_{j \in O} Y_{j,\gamma}^4 \tau_{\alpha,j,i}^7 \quad (2r_T r_V N_o^2) \quad (11843)$$

$$\tau_{\gamma,\delta,w,i}^9 = \sum_{\alpha \in B} \tau_{\gamma,\alpha,i}^8 \tau_{\gamma,\delta,\alpha,w}^6 \quad (2r_D r_T^2 r_V N_o) \quad (11831)$$

$$\tau_{\gamma,\delta,w,i}^9 = \sum_{\alpha \in B} \tau_{\gamma,\alpha,i}^8 \tau_{\gamma,\delta,\alpha,w}^6 \quad (2r_D r_T^2 r_V N_o) \quad (11844)$$

$$\tau_{\gamma,w,i}^{10} = \sum_{\delta \in A} \tau_{\delta,\gamma,w}^0 \tau_{\delta,\gamma,w,i}^9 \quad (2r_D r_T^2 N_o) \quad (11832)$$

$$\tau_{\gamma,w,i}^{10} = \sum_{\delta \in A} \tau_{\delta,\gamma,w}^0 \tau_{\delta,\gamma,w,i}^9 \quad (2r_D r_T^2 N_o) \quad (11845)$$

$${}^2R_{i,\gamma}^4 \leftarrow \sum_{w \in D} \frac{1}{2} {}^2D_{i,w}^4 \tau_{\gamma,w,i}^{10} \quad (2r_D r_T N_o) \quad (11833)$$

$${}^2R_{i,\gamma}^4 \leftarrow \sum_{w \in D} \frac{1}{2} {}^2D_{i,w}^4 \tau_{\gamma,w,i}^{10} \quad (2r_D r_T N_o) \quad (11846)$$

Raw expression

$${}^2R_{j,\zeta}^4 \leftarrow \sum_{\gamma \in A} \sum_{i \in O} \sum_{k \in O} \sum_{l \in O} \sum_{a \in V} \sum_{b \in V} \sum_{c \in V} \frac{1}{2} {}^1T_{b,k} Y_{a,\gamma}^{1,*} Y_{i,\gamma}^{2,*} Z_{\gamma,\zeta}^* Y_{b,\zeta}^{3,*} {}^2D_{a,i,b,j} {}^2T_{c,i,a,l} V_{l,c,k,j} \quad (11834)$$

Factorized expression

$$\tau_{\gamma,\delta,w}^0 = \sum_{a \in V} {}^2D_{a,w}^3 Y_{a,\gamma}^3 Y_{a,\delta}^{3,*} \quad (3r_D r_T^2 N_v) \quad (11835)$$

$$\tau_{\gamma,w,i}^1 = \sum_{a \in V} {}^2D_{a,w}^1 {}^1T_{a,i} Y_{a,\gamma}^{1,*} \quad (3r_D r_T N_o N_v) \quad (11836)$$

Raw expression

$${}^2R_{j,\zeta}^4 \leftarrow \sum_{\gamma \in A} \sum_{i \in O} \sum_{k \in O} \sum_{l \in O} \sum_{a \in V} \sum_{b \in V} \sum_{c \in V} \frac{1}{2} {}^1T_{b,k} Y_{a,\gamma}^{1,*} Y_{i,\gamma}^{2,*} Z_{\gamma,\zeta}^* Y_{b,\zeta}^{3,*} {}^2D_{a,i,b,j} {}^2T_{c,j,a,l} V_{l,i,k,c} \quad (11847)$$

Factorized expression

$$\tau_{\gamma,\delta,w}^0 = \sum_{a \in V} {}^2D_{a,w}^3 Y_{a,\gamma}^1 Y_{a,\delta}^{3,*} \quad (3r_D r_T^2 N_v) \quad (11848)$$

$$\tau_{\gamma,\alpha}^1 = \sum_{i \in O} W_{i,\alpha}^3 Y_{i,\gamma}^2 \quad (2r_T r_V N_o) \quad (11849)$$

$$\tau^2_{\gamma,\alpha} = \sum_{a \in V} W^4_{a,\alpha} Y^3_{a,\gamma} \quad (2r_T r_V N_v) \quad (11850)$$

$$\tau^1_{\gamma,\alpha} = \sum_{a \in V} W^4_{a,\alpha} Y^1_{a,\gamma} \quad (2r_T r_V N_v) \quad (11862)$$

$$\tau^3_{\gamma,\alpha,i} = \sum_{\delta \in A} Z_{\gamma,\delta} Y^4_{i,\delta} \tau^2_{\delta,\alpha} \quad (3r_T^2 r_V N_o) \quad (11851)$$

$$\tau^2_{\gamma,\alpha,i} = \sum_{\delta \in A} Y^2_{i,\delta} Z_{\delta,\gamma} \tau^1_{\delta,\alpha} \quad (3r_T^2 r_V N_o) \quad (11863)$$

$$\tau^4_{\gamma,w,i} = \sum_{a \in V} {}^2D^1_{a,w} {}^1T_{a,i} Y^{1,*}_{a,\gamma} \quad (3r_D r_T N_o N_v) \quad (11852)$$

$$\tau^3_{\gamma,\alpha} = \sum_{i \in O} W^3_{i,\alpha} Y^4_{i,\gamma} \quad (2r_T r_V N_o) \quad (11864)$$

$$\tau^5_{\gamma,\alpha,w} = \sum_{i \in O} W^1_{i,\alpha} \tau^4_{\gamma,w,i} \quad (2r_D r_T r_V N_o) \quad (11853)$$

$$\tau^4_{\gamma,w,i} = \sum_{a \in V} {}^2D^1_{a,w} {}^1T_{a,i} Y^{1,*}_{a,\gamma} \quad (3r_D r_T N_o N_v) \quad (11865)$$

$$\tau^6_{\gamma,\alpha,w} = \sum_{i \in O} {}^2D^2_{i,w} W^2_{i,\alpha} Y^{2,*}_{i,\gamma} \quad (3r_D r_T r_V N_o) \quad (11854)$$

$$\tau^5_{\gamma,\alpha,w} = \sum_{i \in O} W^1_{i,\alpha} \tau^4_{\gamma,w,i} \quad (2r_D r_T r_V N_o) \quad (11866)$$

$$\tau^7_{\gamma,\alpha,w} = \sum_{\beta \in B} X_{\beta,\alpha} \tau^5_{\gamma,\beta,w} \tau^6_{\gamma,\beta,w} \quad (3r_D r_T r_V^2) \quad (11855)$$

$$\tau^6_{\gamma,\alpha,w} = \sum_{i \in O} {}^2D^2_{i,w} W^2_{i,\alpha} Y^{2,*}_{i,\gamma} \quad (3r_D r_T r_V N_o) \quad (11867)$$

$$\tau^8_{\gamma,\alpha,w} = \sum_{\delta \in A} Z^*_{\delta,\gamma} \tau^7_{\delta,\alpha,w} \quad (2r_D r_T^2 r_V) \quad (11856)$$

$$\tau^7_{\gamma,\alpha,w} = \sum_{\beta \in B} X_{\beta,\alpha} \tau^5_{\gamma,\beta,w} \tau^6_{\gamma,\beta,w} \quad (3r_D r_T r_V^2) \quad (11868)$$

$$\tau^9_{\gamma,\delta,w,i} = \sum_{\alpha \in B} \tau^1_{\gamma,\alpha} \tau^3_{\gamma,\alpha,i} \tau^8_{\delta,\alpha,w} \quad (3r_D r_T^2 r_V N_o) \quad (11857)$$

$$\tau^8_{\gamma,\alpha,w} = \sum_{\delta \in A} Z^*_{\delta,\gamma} \tau^7_{\delta,\alpha,w} \quad (2r_D r_T^2 r_V) \quad (11869)$$

$$\tau^{10}_{\gamma,w,i} = \sum_{\delta \in A} \tau^0_{\delta,\gamma,w} \tau^9_{\delta,\gamma,w,i} \quad (2r_D r_T^2 N_o) \quad (11858)$$

$$\tau^9_{\gamma,\delta,w,i} = \sum_{\alpha \in B} \tau^3_{\gamma,\alpha} \tau^2_{\gamma,\alpha,i} \tau^8_{\delta,\alpha,w} \quad (3r_D r_T^2 r_V N_o) \quad (11870)$$

$${}^2R^4_{i,\gamma} \leftarrow \sum_{w \in D} \frac{1}{2} {}^2D^4_{i,w} \tau^{10}_{\gamma,w,i} \quad (2r_D r_T N_o) \quad (11859)$$

$$\tau^{10}_{\gamma,w,i} = \sum_{\delta \in A} \tau^0_{\delta,\gamma,w} \tau^9_{\delta,\gamma,w,i} \quad (2r_D r_T^2 N_o) \quad (11871)$$

Raw expression

$${}^2R^4_{j,\zeta} \leftarrow \sum_{\gamma \in A} \sum_{i \in O} \sum_{k \in O} \sum_{l \in O} \sum_{a \in V} \sum_{b \in V} \sum_{c \in V} \frac{1}{2} {}^1T_{b,k} Y^{1,*}_{a,\gamma} Y^{2,*}_{i,\gamma} Z^*_{\gamma,\zeta} Y^{3,*}_{b,\zeta} {}^2D^{a,i,b,j} {}^2T_{c,l,a,i} V_{k,c,l,j} \quad (11860)$$

Factorized expression

$$\tau^0_{\gamma,\delta,w} = \sum_{a \in V} {}^2D^3_{a,w} Y^3_{a,\gamma} Y^{3,*}_{a,\delta} \quad (3r_D r_T^2 N_v) \quad (11861)$$

$${}^2R^4_{i,\gamma} \leftarrow \sum_{w \in D} \frac{1}{2} {}^2D^4_{i,w} \tau^{10}_{\gamma,w,i} \quad (2r_D r_T N_o) \quad (11872)$$

Raw expression

$${}^2R^4_{j,\zeta} \leftarrow \sum_{\gamma \in A} \sum_{i \in O} \sum_{k \in O} \sum_{l \in O} \sum_{a \in V} \sum_{b \in V} \sum_{c \in V} \frac{1}{2} {}^1T_{c,i} Y^{1,*}_{a,\gamma} Y^{2,*}_{i,\gamma} Z^*_{\gamma,\zeta} Y^{3,*}_{b,\zeta} {}^2D^{a,i,b,j} {}^2T_{a,k,b,l} V_{k,c,l,j} \quad (11873)$$

Factorized expression

$$\tau^0_{\gamma,\delta,w} = \sum_{a \in V} {}^2D^3_{a,w} Y^1_{a,\gamma} Y^{3,*}_{a,\delta} \quad (3r_D r_T^2 N_v) \quad (11874)$$

$$\tau^1_{\gamma,w,i} = \sum_{a \in V} {}^2D^1_{a,w} {}^1T_{a,i} Y^{1,*}_{a,\gamma} \quad (3r_D r_T N_o N_v) \quad (11886)$$

$$\tau^1_{\gamma,w,i} = \sum_{a \in V} {}^2D^1_{a,w} {}^1T_{a,i} Y^{1,*}_{a,\gamma} \quad (3r_D r_T N_o N_v) \quad (11875)$$

$$\tau^2_{\alpha,i,j} = \sum_{\beta \in B} W^1_{i,\beta} W^2_{j,\beta} X_{\beta,\alpha} \quad (3r_V^2 N_o^2) \quad (11887)$$

$$\tau^2_{\alpha,i,j} = \sum_{\beta \in B} W^1_{i,\beta} W^2_{j,\beta} X_{\beta,\alpha} \quad (3r_V^2 N_o^2) \quad (11876)$$

$$\tau^3_{\gamma,\alpha,i} = \sum_{j \in O} Y^2_{j,\gamma} \tau^2_{\alpha,j,i} \quad (2r_T r_V N_o^2) \quad (11888)$$

$$\tau^3_{\gamma,\alpha,i} = \sum_{j \in O} Y^4_{j,\gamma} \tau^2_{\alpha,j,i} \quad (2r_T r_V N_o^2) \quad (11877)$$

$$\tau^4_{\gamma,\alpha} = \sum_{a \in V} W^4_{a,\alpha} Y^1_{a,\gamma} \quad (2r_T r_V N_v) \quad (11889)$$

$$\tau^4_{\gamma,\alpha} = \sum_{a \in V} W^4_{a,\alpha} Y^3_{a,\gamma} \quad (2r_T r_V N_v) \quad (11878)$$

$$\tau^5_{\gamma,i,j} = \sum_{\alpha \in B} W^3_{j,\alpha} \tau^4_{\gamma,\alpha} \tau^3_{\gamma,\alpha,i} \quad (3r_T r_V N_o^2) \quad (11890)$$

$$\tau^5_{\gamma,i,j} = \sum_{\alpha \in B} W^3_{j,\alpha} \tau^4_{\gamma,\alpha} \tau^3_{\gamma,\alpha,i} \quad (3r_T r_V N_o^2) \quad (11879)$$

$$\tau^6_{\gamma,i,j} = \sum_{\delta \in A} Z_{\delta,\gamma} \tau^5_{\delta,i,j} \quad (2r_T^2 N_o^2) \quad (11891)$$

$$\tau^6_{\gamma,i,j} = \sum_{\delta \in A} Z_{\gamma,\delta} \tau^5_{\delta,i,j} \quad (2r_T^2 N_o^2) \quad (11880)$$

$$\tau^7_{\gamma,\delta,w} = \sum_{i \in O} \sum_{j \in O} {}^2D^2_{i,w} Y^{2,*}_{i,\delta} \tau^1_{\delta,w,j} \tau^6_{\gamma,i,j} \quad (4r_D r_T^2 N_o^2) \quad (11892)$$

$$\tau^7_{\gamma,\delta,w} = \sum_{i \in O} \sum_{j \in O} {}^2D^2_{i,w} Y^{2,*}_{i,\delta} \tau^1_{\delta,w,j} \tau^6_{\gamma,i,j} \quad (4r_D r_T^2 N_o^2) \quad (11881)$$

$$\tau^8_{\gamma,\delta,w} = \sum_{\epsilon \in A} Z^*_{\epsilon,\delta} \tau^7_{\gamma,\epsilon,w} \quad (2r_D r_T^3) \quad (11893)$$

$$\tau^8_{\gamma,\delta,w} = \sum_{\epsilon \in A} Z^*_{\epsilon,\delta} \tau^7_{\gamma,\epsilon,w} \quad (2r_D r_T^3) \quad (11882)$$

$${}^2R^4_{i,\gamma} \leftarrow \sum_{\delta \in A} \sum_{w \in D} \frac{1}{2} {}^2D^4_{i,w} Y^4_{i,\delta} \tau^0_{\delta,\gamma,w} \tau^8_{\delta,\gamma,w} \quad (4r_D r_T^2 N_o) \quad (11894)$$

$${}^2R^4_{i,\gamma} \leftarrow \sum_{\delta \in A} \sum_{w \in D} \frac{1}{2} {}^2D^4_{i,w} Y^2_{i,\delta} \tau^0_{\delta,\gamma,w} \tau^8_{\delta,\gamma,w} \quad (4r_D r_T^2 N_o) \quad (11883)$$

Raw expression

Raw expression

$${}^2R^4_{j,\zeta} \leftarrow \sum_{\gamma \in A} \sum_{i \in O} \sum_{k \in O} \sum_{l \in O} \sum_{a \in V} \sum_{b \in V} \sum_{c \in V} \frac{1}{2} {}^1T_{c,j} Y^{1,*}_{a,\gamma} Y^{2,*}_{i,\gamma} Z^*_{\gamma,\zeta} Y^{3,*}_{b,\zeta} {}^2D^{a,i,b,j} {}^2T_{a,k,b,l} V_{k,i,l,c} \quad (11895)$$

$${}^2R^4_{j,\zeta} \leftarrow \sum_{\gamma \in A} \sum_{i \in O} \sum_{k \in O} \sum_{l \in O} \sum_{a \in V} \sum_{b \in V} \sum_{c \in V} \frac{1}{2} {}^1T_{c,i} Y^{1,*}_{a,\gamma} Y^{2,*}_{i,\gamma} Z^*_{\gamma,\zeta} Y^{3,*}_{b,\zeta} {}^2D^{a,i,b,j} {}^2T_{b,k,a,l} V_{l,c,k,j} \quad (11884)$$

Factorized expression

Factorized expression

$$\tau^0_{\gamma,\delta,w} = \sum_{a \in V} {}^2D^3_{a,w} {}^1T_{a,i} Y^{3,*}_{a,\gamma} \quad (3r_D r_T N_o N_v) \quad (11896)$$

$$\tau^0_{\gamma,\delta,w} = \sum_{a \in V} {}^2D^3_{a,w} Y^3_{a,\gamma} Y^{3,*}_{a,\delta} \quad (3r_D r_T^2 N_v) \quad (11885)$$

$$\tau^1_{\gamma,\alpha} = \sum_{a \in V} W^2_{a,\alpha} Y^3_{a,\gamma} \quad (2r_T r_V N_v) \quad (11897)$$

$$\tau^2_{\alpha,i,j} = \sum_{\beta \in B} X_{\alpha,\beta} W^3_{i,\beta} W^4_{j,\beta} \quad (3r_V^2 N_o^2) \quad (11898)$$

$$\tau^2_{\alpha,i,j} = \sum_{\beta \in B} X_{\alpha,\beta} W^3_{i,\beta} W^4_{j,\beta} \quad (3r_V^2 N_o^2) \quad (11911)$$

$$\tau^3_{\gamma,\alpha,i} = \sum_{j \in O} Y^4_{j,\gamma} \tau^2_{\alpha,j,i} \quad (2r_T r_V N_o^2) \quad (11899)$$

$$\tau^3_{\gamma,\alpha,i} = \sum_{j \in O} Y^2_{j,\gamma} \tau^2_{\alpha,j,i} \quad (2r_T r_V N_o^2) \quad (11912)$$

$$\tau^4_{\gamma,i,j} = \sum_{\alpha \in B} W^1_{i,\alpha} \tau^1_{\gamma,\alpha} \tau^3_{\gamma,\alpha,j} \quad (3r_T r_V N_o^2) \quad (11900)$$

$$\tau^4_{\gamma,i,j} = \sum_{\alpha \in B} W^1_{i,\alpha} \tau^1_{\gamma,\alpha} \tau^3_{\gamma,\alpha,j} \quad (3r_T r_V N_o^2) \quad (11913)$$

$$\tau^5_{\gamma,i,j} = \sum_{\delta \in A} Z_{\gamma,\delta} \tau^4_{\delta,i,j} \quad (2r_T^2 N_o^2) \quad (11901)$$

$$\tau^5_{\gamma,i,j} = \sum_{\delta \in A} Z_{\delta,\gamma} \tau^4_{\delta,i,j} \quad (2r_T^2 N_o^2) \quad (11914)$$

$$\tau^6_{\gamma,\delta,w} = \sum_{a \in V} {}^2D^1_{a,w} Y^1_{a,\gamma} Y^{1,*}_{a,\delta} \quad (3r_D r_T^2 N_v) \quad (11902)$$

$$\tau^6_{\gamma,\delta,w} = \sum_{a \in V} {}^2D^1_{a,w} Y^3_{a,\gamma} Y^{1,*}_{a,\delta} \quad (3r_D r_T^2 N_v) \quad (11915)$$

$$\tau^7_{\gamma,\delta,w} = \sum_{i \in O} {}^2D^2_{i,w} Y^2_{i,\gamma} Y^{2,*}_{i,\delta} \quad (3r_D r_T^2 N_o) \quad (11903)$$

$$\tau^7_{\gamma,\delta,w} = \sum_{i \in O} {}^2D^2_{i,w} Y^4_{i,\gamma} Y^{2,*}_{i,\delta} \quad (3r_D r_T^2 N_o) \quad (11916)$$

$$\tau^8_{\gamma,\delta,w} = \sum_{\epsilon \in A} Z^*_{\epsilon,\delta} \tau^6_{\gamma,\epsilon,w} \tau^7_{\gamma,\epsilon,w} \quad (3r_D r_T^3) \quad (11904)$$

$$\tau^8_{\gamma,\delta,w} = \sum_{\epsilon \in A} Z^*_{\epsilon,\delta} \tau^6_{\gamma,\epsilon,w} \tau^7_{\gamma,\epsilon,w} \quad (3r_D r_T^3) \quad (11917)$$

$$\tau^9_{\gamma,w,i,j} = \sum_{\delta \in A} \tau^5_{\delta,i,j} \tau^8_{\delta,\gamma,w} \quad (2r_D r_T^2 N_o^2) \quad (11905)$$

$$\tau^9_{\gamma,w,i,j} = \sum_{\delta \in A} \tau^5_{\delta,i,j} \tau^8_{\delta,\gamma,w} \quad (2r_D r_T^2 N_o^2) \quad (11918)$$

$$\tau^{10}_{\gamma,w,i} = \sum_{j \in O} \tau^0_{\gamma,w,j} \tau^9_{\gamma,w,j,i} \quad (2r_D r_T N_o^2) \quad (11906)$$

$$\tau^{10}_{\gamma,w,i} = \sum_{j \in O} \tau^0_{\gamma,w,j} \tau^9_{\gamma,w,j,i} \quad (2r_D r_T N_o^2) \quad (11919)$$

$${}^2R^4_{i,\gamma} \leftarrow \sum_{w \in D} \frac{1}{2} {}^2D^4_{i,w} \tau^{10}_{\gamma,w,i} \quad (2r_D r_T N_o) \quad (11907)$$

$${}^2R^4_{i,\gamma} \leftarrow \sum_{w \in D} \frac{1}{2} {}^2D^4_{i,w} \tau^{10}_{\gamma,w,i} \quad (2r_D r_T N_o) \quad (11920)$$

Raw expression

$${}^2R^4_{j,\zeta} \leftarrow \sum_{\gamma \in A} \sum_{i \in O} \sum_{k \in O} \sum_{l \in O} \sum_{a \in V} \sum_{b \in V} \sum_{c \in V} \frac{1}{2} {}^1T_{c,j} Y^{1,*}_{a,\gamma} Y^{2,*}_{i,\gamma} Z^*_{\gamma,\zeta} Y^{3,*}_{b,\zeta} {}^2D^{a,i,b,j} {}^2T_{b,k,a,l} V_{l,i,k,c} \quad (11908)$$

Raw expression

$${}^2R^4_{j,\zeta} \leftarrow \sum_{\gamma \in A} \sum_{i \in O} \sum_{k \in O} \sum_{l \in O} \sum_{a \in V} \sum_{b \in V} \sum_{c \in V} \frac{1}{2} {}^1T_{c,k} Y^{1,*}_{a,\gamma} Y^{2,*}_{i,\gamma} Z^*_{\gamma,\zeta} Y^{3,*}_{b,\zeta} {}^2D^{a,i,b,j} {}^2T_{a,i,b,l} V_{l,c,k,j} \quad (11921)$$

Factorized expression

$$\tau^0_{\gamma,w,i} = \sum_{a \in V} {}^2D^3_{a,w} {}^1T_{a,i} Y^{3,*}_{a,\gamma} \quad (3r_D r_T N_o N_v) \quad (11909)$$

Factorized expression

$$\tau^0_{\gamma,\delta,w} = \sum_{a \in V} {}^2D^1_{a,w} Y^1_{a,\gamma} Y^{1,*}_{a,\delta} \quad (3r_D r_T^2 N_v) \quad (11922)$$

$$\tau^1_{\gamma,\alpha} = \sum_{a \in V} W^2_{a,\alpha} Y^1_{a,\gamma} \quad (2r_T r_V N_v) \quad (11910)$$

$$\tau^1_{\gamma,\alpha} = \sum_{i \in O} W^1_{i,\alpha} Y^2_{i,\gamma} \quad (2r_T r_V N_o) \quad (11923)$$

$$\tau^2_{\gamma,\alpha} = \sum_{a \in V} W^2_{a,\alpha} Y^3_{a,\gamma} \quad (2r_T r_V N_v) \quad (11924)$$

$$\tau^2_{\gamma,\alpha,i} = \sum_{\delta \in A} Y^2_{i,\delta} Z_{\delta,\gamma} \tau^1_{\delta,\alpha} \quad (3r_T^2 r_V N_o) \quad (11936)$$

$$\tau^3_{\gamma,\alpha,i} = \sum_{\delta \in A} Z_{\gamma,\delta} Y^4_{i,\delta} \tau^2_{\delta,\alpha} \quad (3r_T^2 r_V N_o) \quad (11925)$$

$$\tau^3_{\gamma,\alpha} = \sum_{i \in O} W^1_{i,\alpha} Y^4_{i,\gamma} \quad (2r_T r_V N_o) \quad (11937)$$

$$\tau^4_{\gamma,\alpha,w} = \sum_{\delta \in A} \sum_{i \in O} {}^2D^2_{i,w} Y^{2,*}_{i,\gamma} \tau^1_{\delta,\alpha} \tau^0_{\delta,\gamma,w} \tau^3_{\delta,\alpha,i} \quad (5r_D r_T^2 r_V N_o) \quad (11926)$$

$$\tau^4_{\gamma,\alpha,w} = \sum_{\delta \in A} \sum_{i \in O} {}^2D^2_{i,w} Y^{2,*}_{i,\gamma} \tau^3_{\delta,\alpha} \tau^0_{\delta,\gamma,w} \tau^2_{\delta,\alpha,i} \quad (5r_D r_T^2 r_V N_o) \quad (11938)$$

$$\tau^5_{\gamma,\alpha,w} = \sum_{\beta \in B} X_{\beta,\alpha} \tau^4_{\gamma,\beta,w} \quad (2r_D r_T r_V^2) \quad (11927)$$

$$\tau^5_{\gamma,\alpha,w} = \sum_{\beta \in B} X_{\beta,\alpha} \tau^4_{\gamma,\beta,w} \quad (2r_D r_T r_V^2) \quad (11939)$$

$$\tau^6_{\gamma,\alpha,w} = \sum_{\delta \in A} Z^*_{\delta,\gamma} \tau^5_{\delta,\alpha,w} \quad (2r_D r_T^2 r_V) \quad (11928)$$

$$\tau^6_{\gamma,\alpha,w} = \sum_{\delta \in A} Z^*_{\delta,\gamma} \tau^5_{\delta,\alpha,w} \quad (2r_D r_T^2 r_V) \quad (11940)$$

$$\tau^7_{\gamma,w,i} = \sum_{a \in V} {}^2D^3_{a,w} {}^1T_{a,i} Y^{3,*}_{a,\gamma} \quad (3r_D r_T N_o N_v) \quad (11929)$$

$$\tau^7_{\gamma,w,i} = \sum_{a \in V} {}^2D^3_{a,w} {}^1T_{a,i} Y^{3,*}_{a,\gamma} \quad (3r_D r_T N_o N_v) \quad (11941)$$

$$\tau^8_{\gamma,\alpha,w} = \sum_{i \in O} W^3_{i,\alpha} \tau^7_{\gamma,w,i} \quad (2r_D r_T r_V N_o) \quad (11930)$$

$$\tau^8_{\gamma,\alpha,w} = \sum_{i \in O} W^3_{i,\alpha} \tau^7_{\gamma,w,i} \quad (2r_D r_T r_V N_o) \quad (11942)$$

$$\tau^9_{\gamma,w,i} = \sum_{\alpha \in B} W^4_{i,\alpha} \tau^6_{\gamma,\alpha,w} \tau^8_{\gamma,\alpha,w} \quad (3r_D r_T r_V N_o) \quad (11931)$$

$$\tau^9_{\gamma,w,i} = \sum_{\alpha \in B} W^4_{i,\alpha} \tau^6_{\gamma,\alpha,w} \tau^8_{\gamma,\alpha,w} \quad (3r_D r_T r_V N_o) \quad (11943)$$

$${}^2R^4_{i,\gamma} \leftarrow \sum_{w \in D} \frac{1}{2} {}^2D^4_{i,w} \tau^9_{\gamma,w,i} \quad (2r_D r_T N_o) \quad (11932)$$

$${}^2R^4_{i,\gamma} \leftarrow \sum_{w \in D} \frac{1}{2} {}^2D^4_{i,w} \tau^9_{\gamma,w,i} \quad (2r_D r_T N_o) \quad (11944)$$

Raw expression

$${}^2R^4_{j,\zeta} \leftarrow \sum_{\gamma \in A} \sum_{i \in O} \sum_{k \in O} \sum_{l \in O} \sum_{a \in V} \sum_{b \in V} \sum_{c \in V} \frac{1}{2} {}^1T_{c,k} Y^{1,*}_{a,\gamma} Y^{2,*}_{i,\gamma} Z^*_{\gamma,\zeta} Y^{3,*}_{b,\zeta} {}^2D^{a,i,b,j} {}^2T_{a,l,b,j} V_{k,i,l,c} \quad (11933)$$

Raw expression

$${}^2R^4_{j,\zeta} \leftarrow \sum_{\gamma \in A} \sum_{i \in O} \sum_{k \in O} \sum_{l \in O} \sum_{a \in V} \sum_{b \in V} \sum_{c \in V} \frac{1}{2} {}^1T_{c,k} Y^{1,*}_{a,\gamma} Y^{2,*}_{i,\gamma} Z^*_{\gamma,\zeta} Y^{3,*}_{b,\zeta} {}^2D^{a,i,b,j} {}^2T_{b,j,a,l} V_{k,i,l,c} \quad (11945)$$

Factorized expression

$$\tau^0_{\gamma,\delta,w} = \sum_{a \in V} {}^2D^1_{a,w} Y^3_{a,\gamma} Y^{1,*}_{a,\delta} \quad (3r_D r_T^2 N_v) \quad (11934)$$

Factorized expression

$$\tau^0_{\gamma,w,i} = \sum_{a \in V} {}^2D^3_{a,w} {}^1T_{a,i} Y^{3,*}_{a,\gamma} \quad (3r_D r_T N_o N_v) \quad (11946)$$

$$\tau^1_{\gamma,\alpha} = \sum_{a \in V} W^2_{a,\alpha} Y^1_{a,\gamma} \quad (2r_T r_V N_v) \quad (11935)$$

$$\tau^1_{\gamma,\delta,w} = \sum_{a \in V} {}^2D^1_{a,w} Y^1_{a,\gamma} Y^{1,*}_{a,\delta} \quad (3r_D r_T^2 N_v) \quad (11947)$$

$$\tau_{\alpha,i,j}^2 = \sum_{\beta \in B} W_{i,\beta}^1 W_{j,\beta}^2 X_{\beta,\alpha} \quad (3r_V^2 N_o^2) \quad (11948)$$

$$\tau_{\alpha,i,j}^2 = \sum_{\beta \in B} W_{i,\beta}^1 W_{j,\beta}^2 X_{\beta,\alpha} \quad (3r_V^2 N_o^2) \quad (11961)$$

$$\tau_{\gamma,\alpha,i}^3 = \sum_{j \in O} Y_{j,\gamma}^2 \tau_{\alpha,j,i}^2 \quad (2r_T r_V N_o^2) \quad (11949)$$

$$\tau_{\gamma,\alpha,i}^3 = \sum_{j \in O} Y_{j,\gamma}^4 \tau_{\alpha,j,i}^2 \quad (2r_T r_V N_o^2) \quad (11962)$$

$$\tau_{\gamma,\delta,\alpha,w}^4 = \sum_{i \in O} {}^2D_{i,w}^2 Y_{i,\delta}^{2,*} \tau_{\gamma,\delta,w}^1 \tau_{\gamma,\alpha,i}^3 \quad (4r_D r_T^2 r_V N_o) \quad (11950)$$

$$\tau_{\gamma,\delta,\alpha,w}^4 = \sum_{i \in O} {}^2D_{i,w}^2 Y_{i,\delta}^{2,*} \tau_{\gamma,\delta,w}^1 \tau_{\gamma,\alpha,i}^3 \quad (4r_D r_T^2 r_V N_o) \quad (11963)$$

$$\tau_{\gamma,\alpha}^5 = \sum_{a \in V} W_{a,\alpha}^4 Y_{a,\gamma}^3 \quad (2r_T r_V N_v) \quad (11951)$$

$$\tau_{\gamma,\alpha}^5 = \sum_{a \in V} W_{a,\alpha}^4 Y_{a,\gamma}^1 \quad (2r_T r_V N_v) \quad (11964)$$

$$\tau_{\gamma,\alpha,i}^6 = \sum_{\delta \in A} Z_{\gamma,\delta} Y_{i,\delta}^4 \tau_{\delta,\alpha}^5 \quad (3r_T^2 r_V N_o) \quad (11952)$$

$$\tau_{\gamma,\alpha,i}^6 = \sum_{\delta \in A} Y_{i,\delta}^2 Z_{\delta,\gamma} \tau_{\delta,\alpha}^5 \quad (3r_T^2 r_V N_o) \quad (11965)$$

$$\tau_{\gamma,\alpha,w,i}^7 = \sum_{\delta \in A} \tau_{\delta,\alpha,i}^6 \tau_{\delta,\gamma,\alpha,w}^4 \quad (2r_D r_T^2 r_V N_o) \quad (11953)$$

$$\tau_{\gamma,\alpha,w,i}^7 = \sum_{\delta \in A} \tau_{\delta,\alpha,i}^6 \tau_{\delta,\gamma,\alpha,w}^4 \quad (2r_D r_T^2 r_V N_o) \quad (11966)$$

$$\tau_{\gamma,w,i,j}^8 = \sum_{\alpha \in B} W_{i,\alpha}^3 \tau_{\gamma,\alpha,w,j}^7 \quad (2r_D r_T r_V N_o^2) \quad (11954)$$

$$\tau_{\gamma,w,i,j}^8 = \sum_{\alpha \in B} W_{i,\alpha}^3 \tau_{\gamma,\alpha,w,j}^7 \quad (2r_D r_T r_V N_o^2) \quad (11967)$$

$$\tau_{\gamma,w,i,j}^9 = \sum_{\delta \in A} Z_{\delta,\gamma}^* \tau_{\delta,w,i,j}^8 \quad (2r_D r_T^2 N_o^2) \quad (11955)$$

$$\tau_{\gamma,w,i,j}^9 = \sum_{\delta \in A} Z_{\delta,\gamma}^* \tau_{\delta,w,i,j}^8 \quad (2r_D r_T^2 N_o^2) \quad (11968)$$

$$\tau_{\gamma,w,i}^{10} = \sum_{j \in O} \tau_{\gamma,w,j}^0 \tau_{\gamma,w,j,i}^9 \quad (2r_D r_T N_o^2) \quad (11956)$$

$$\tau_{\gamma,w,i}^{10} = \sum_{j \in O} \tau_{\gamma,w,j}^0 \tau_{\gamma,w,j,i}^9 \quad (2r_D r_T N_o^2) \quad (11969)$$

$${}^2R_{i,\gamma}^4 \leftarrow \sum_{w \in D} \frac{1}{2} {}^2D_{i,w}^4 \tau_{\gamma,w,i}^{10} \quad (2r_D r_T N_o) \quad (11957)$$

$${}^2R_{i,\gamma}^4 \leftarrow \sum_{w \in D} \frac{1}{2} {}^2D_{i,w}^4 \tau_{\gamma,w,i}^{10} \quad (2r_D r_T N_o) \quad (11970)$$

Raw expression

$${}^2R_{j,\zeta}^4 \leftarrow \sum_{\gamma \in A} \sum_{i \in O} \sum_{k \in O} \sum_{l \in O} \sum_{a \in V} \sum_{b \in V} \sum_{c \in V} \frac{1}{2} {}^1T_{c,k} Y_{a,\gamma}^{1,*} Y_{i,\gamma}^{2,*} Z_{\gamma,\zeta}^* Y_{b,\zeta}^{3,*} {}^2D_{a,i,b,j} {}^2T_{b,l,a,i} V_{l,c,k,j} \quad (11958)$$

Factorized expression

$$\tau_{\gamma,w,i}^0 = \sum_{a \in V} {}^2D_{a,w}^3 {}^1T_{a,i} Y_{a,\gamma}^{3,*} \quad (3r_D r_T N_o N_v) \quad (11959)$$

$$\tau_{\gamma,\delta,w}^1 = \sum_{a \in V} {}^2D_{a,w}^1 Y_{a,\gamma}^3 Y_{a,\delta}^{1,*} \quad (3r_D r_T^2 N_v) \quad (11960)$$

Raw expression

$${}^2R_{j,\zeta}^4 \leftarrow - \sum_{\gamma \in A} \sum_{i \in O} \sum_{k \in O} \sum_{l \in O} \sum_{a \in V} \sum_{b \in V} \sum_{c \in V} {}^1T_{a,k} Y_{a,\gamma}^{1,*} Y_{i,\gamma}^{2,*} Z_{\gamma,\zeta}^* Y_{b,\zeta}^{3,*} {}^2D_{a,i,b,j} {}^2T_{b,j,c,l} V_{k,i,l,c} \quad (11971)$$

Factorized expression

$$\tau_{\gamma,\delta,w}^0 = \sum_{a \in V} {}^2D_{a,w}^3 Y_{a,\gamma}^3 Y_{a,\delta}^{3,*} \quad (3r_D r_T^2 N_v) \quad (11972)$$

$$\tau_{\alpha,i}^1 = \sum_{a \in V} {}^1T_{a,i} W_{a,\alpha}^2 \quad (2r_V N_o N_v) \quad (11973)$$



$$\tau^2_{\gamma,\alpha,w} = \sum_{i \in O} {}^2D^2_{i,w} Y^{2,*}_{i,\gamma} \tau^1_{\alpha,i} \quad (3r_D r_T r_V N_o) \quad (11974)$$

$$\tau^2_{\gamma,\alpha,w} = \sum_{i \in O} {}^2D^2_{i,w} Y^{2,*}_{i,\gamma} \tau^1_{\alpha,i} \quad (3r_D r_T r_V N_o) \quad (11986)$$

$$\tau^3_{\gamma,\delta,w} = \sum_{a \in V} {}^2D^1_{a,w} Y^1_{a,\gamma} Y^{1,*}_{a,\delta} \quad (3r_D r_T^2 N_v) \quad (11975)$$

$$\tau^3_{\gamma,\delta,w} = \sum_{a \in V} {}^2D^1_{a,w} Y^3_{a,\gamma} Y^{1,*}_{a,\delta} \quad (3r_D r_T^2 N_v) \quad (11987)$$

$$\tau^4_{\gamma,\delta,w,i} = \sum_{\epsilon \in A} Y^2_{i,\epsilon} Z_{\epsilon,\gamma} \tau^3_{\epsilon,\delta,w} \quad (3r_D r_T^3 N_o) \quad (11976)$$

$$\tau^4_{\gamma,\delta,w,i} = \sum_{\epsilon \in A} Z_{\gamma,\epsilon} Y^4_{i,\epsilon} \tau^3_{\epsilon,\delta,w} \quad (3r_D r_T^3 N_o) \quad (11988)$$

$$\tau^5_{\gamma,\delta,\alpha,w} = \sum_{i \in O} W^1_{i,\alpha} \tau^2_{\delta,\alpha,w} \tau^4_{\gamma,\delta,w,i} \quad (3r_D r_T^2 r_V N_o) \quad (11977)$$

$$\tau^5_{\gamma,\delta,\alpha,w} = \sum_{i \in O} W^1_{i,\alpha} \tau^2_{\delta,\alpha,w} \tau^4_{\gamma,\delta,w,i} \quad (3r_D r_T^2 r_V N_o) \quad (11989)$$

$$\tau^6_{\alpha,i,j} = \sum_{\beta \in B} X_{\alpha,\beta} W^3_{i,\beta} W^4_{j,\beta} \quad (3r_V^2 N_o^2) \quad (11978)$$

$$\tau^6_{\alpha,i,j} = \sum_{\beta \in B} X_{\alpha,\beta} W^3_{i,\beta} W^4_{j,\beta} \quad (3r_V^2 N_o^2) \quad (11990)$$

$$\tau^7_{\gamma,\alpha,i} = \sum_{j \in O} Y^4_{j,\gamma} \tau^6_{\alpha,j,i} \quad (2r_T r_V N_o^2) \quad (11979)$$

$$\tau^7_{\gamma,\alpha,i} = \sum_{j \in O} Y^2_{j,\gamma} \tau^6_{\alpha,j,i} \quad (2r_T r_V N_o^2) \quad (11991)$$

$$\tau^8_{\gamma,\delta,w,i} = \sum_{\alpha \in B} \tau^7_{\gamma,\alpha,i} \tau^5_{\gamma,\delta,\alpha,w} \quad (2r_D r_T^2 r_V N_o) \quad (11980)$$

$$\tau^8_{\gamma,\delta,w,i} = \sum_{\alpha \in B} \tau^7_{\gamma,\alpha,i} \tau^5_{\gamma,\delta,\alpha,w} \quad (2r_D r_T^2 r_V N_o) \quad (11992)$$

$$\tau^9_{\gamma,\delta,i} = \sum_{\epsilon \in A} \sum_{w \in D} {}^2D^4_{i,w} \tau^0_{\epsilon,\delta,w} \tau^8_{\epsilon,\gamma,w,i} \quad (3r_D r_T^3 N_o) \quad (11981)$$

$$\tau^9_{\gamma,\delta,i} = \sum_{\epsilon \in A} \sum_{w \in D} {}^2D^4_{i,w} \tau^0_{\epsilon,\delta,w} \tau^8_{\epsilon,\gamma,w,i} \quad (3r_D r_T^3 N_o) \quad (11993)$$

$${}^2R^4_{i,\gamma} \leftarrow \sum_{\delta \in A} \frac{1}{2} Z^*_{\delta,\gamma} \tau^9_{\delta,\gamma,i} \quad (2r_T^2 N_o) \quad (11982)$$

$${}^2R^4_{i,\gamma} \leftarrow \sum_{\delta \in A} \frac{1}{2} Z^*_{\delta,\gamma} \tau^9_{\delta,\gamma,i} \quad (2r_T^2 N_o) \quad (11994)$$

Raw expression

$${}^2R^4_{j,\zeta} \leftarrow - \sum_{\gamma \in A} \sum_{i \in O} \sum_{k \in O} \sum_{l \in O} \sum_{a \in V} \sum_{b \in V} \sum_{c \in V} {}^1T_{a,k} Y^{1,*}_{a,\gamma} Y^{2,*}_{i,\gamma} Z^*_{\gamma,\zeta} Y^{3,*}_{b,\zeta} {}^2D^{a,i,b,j} {}^2T_{c,l,b,j} V_{k,i,l,c} \quad (11983)$$

Raw expression

$${}^2R^4_{j,\zeta} \leftarrow - \sum_{\gamma \in A} \sum_{i \in O} \sum_{k \in O} \sum_{l \in O} \sum_{a \in V} \sum_{b \in V} \sum_{c \in V} {}^1T_{b,k} Y^{1,*}_{a,\gamma} Y^{2,*}_{i,\gamma} Z^*_{\gamma,\zeta} Y^{3,*}_{b,\zeta} {}^2D^{a,i,b,j} {}^2T_{a,i,c,l} V_{l,c,k,j} \quad (11995)$$

Factorized expression

$$\tau^0_{\gamma,\delta,w} = \sum_{a \in V} {}^2D^3_{a,w} Y^1_{a,\gamma} Y^{3,*}_{a,\delta} \quad (3r_D r_T^2 N_v) \quad (11984)$$

$$\tau^0_{\gamma,\delta,w} = \sum_{a \in V} {}^2D^3_{a,w} Y^3_{a,\gamma} Y^{3,*}_{a,\delta} \quad (3r_D r_T^2 N_v) \quad (11996)$$

$$\tau^1_{\alpha,i} = \sum_{a \in V} {}^1T_{a,i} W^2_{a,\alpha} \quad (2r_V N_o N_v) \quad (11985)$$

$$\tau^1_{\gamma,\alpha,w} = \sum_{i \in O} {}^2D^2_{i,w} W^2_{i,\alpha} Y^{2,*}_{i,\gamma} \quad (3r_D r_T r_V N_o) \quad (11997)$$

$$\tau^2_{\gamma,\delta,w} = \sum_{a \in V} {}^2D^1_{a,w} Y^1_{a,\gamma} Y^{1,*}_{a,\delta} \quad (3r_D r_T^2 N_v) \quad (11998)$$

$$\tau^2_{\gamma,\delta,w} = \sum_{a \in V} {}^2D^1_{a,w} Y^3_{a,\gamma} Y^{1,*}_{a,\delta} \quad (3r_D r_T^2 N_v) \quad (12010)$$

$$\tau^3_{\gamma,\delta,w,i} = \sum_{\epsilon \in A} Y^2_{i,\epsilon} Z_{\epsilon,\gamma} \tau^2_{\epsilon,\delta,w} \quad (3r_D r_T^3 N_o) \quad (11999)$$

$$\tau^3_{\gamma,\delta,w,i} = \sum_{\epsilon \in A} Z_{\gamma,\epsilon} Y^4_{i,\epsilon} \tau^2_{\epsilon,\delta,w} \quad (3r_D r_T^3 N_o) \quad (12011)$$

$$\tau^4_{\gamma,\delta,\alpha,w} = \sum_{i \in O} W^1_{i,\alpha} \tau^1_{\delta,\alpha,w} \tau^3_{\gamma,\delta,w,i} \quad (3r_D r_T^2 r_V N_o) \quad (12000)$$

$$\tau^4_{\gamma,\delta,\alpha,w} = \sum_{i \in O} W^1_{i,\alpha} \tau^1_{\delta,\alpha,w} \tau^3_{\gamma,\delta,w,i} \quad (3r_D r_T^2 r_V N_o) \quad (12012)$$

$$\tau^5_{\alpha,i} = \sum_{a \in V} {}^1T_{a,i} W^4_{a,\alpha} \quad (2r_V N_o N_v) \quad (12001)$$

$$\tau^5_{\alpha,i} = \sum_{a \in V} {}^1T_{a,i} W^4_{a,\alpha} \quad (2r_V N_o N_v) \quad (12013)$$

$$\tau^6_{\alpha,i,j} = \sum_{\beta \in B} X_{\alpha,\beta} W^3_{j,\beta} \tau^5_{\beta,i} \quad (3r_V^2 N_o^2) \quad (12002)$$

$$\tau^6_{\alpha,i,j} = \sum_{\beta \in B} X_{\alpha,\beta} W^3_{j,\beta} \tau^5_{\beta,i} \quad (3r_V^2 N_o^2) \quad (12014)$$

$$\tau^7_{\gamma,\alpha,i} = \sum_{j \in O} Y^4_{j,\gamma} \tau^6_{\alpha,i,j} \quad (2r_T r_V N_o^2) \quad (12003)$$

$$\tau^7_{\gamma,\alpha,i} = \sum_{j \in O} Y^2_{j,\gamma} \tau^6_{\alpha,i,j} \quad (2r_T r_V N_o^2) \quad (12015)$$

$$\tau^8_{\gamma,\delta,w,i} = \sum_{\alpha \in B} \tau^7_{\gamma,\alpha,i} \tau^4_{\gamma,\delta,\alpha,w} \quad (2r_D r_T^2 r_V N_o) \quad (12004)$$

$$\tau^8_{\gamma,\delta,w,i} = \sum_{\alpha \in B} \tau^7_{\gamma,\alpha,i} \tau^4_{\gamma,\delta,\alpha,w} \quad (2r_D r_T^2 r_V N_o) \quad (12016)$$

$$\tau^9_{\gamma,\delta,i} = \sum_{\epsilon \in A} \sum_{w \in D} {}^2D^4_{i,w} \tau^0_{\epsilon,\delta,w} \tau^8_{\epsilon,\gamma,w,i} \quad (3r_D r_T^3 N_o) \quad (12005)$$

$$\tau^9_{\gamma,\delta,i} = \sum_{\epsilon \in A} \sum_{w \in D} {}^2D^4_{i,w} \tau^0_{\epsilon,\delta,w} \tau^8_{\epsilon,\gamma,w,i} \quad (3r_D r_T^3 N_o) \quad (12017)$$

$${}^2R^4_{i,\gamma} \leftarrow \sum_{\delta \in A} \frac{1}{2} Z^*_{\delta,\gamma} \tau^9_{\delta,\gamma,i} \quad (2r_T^2 N_o) \quad (12006)$$

$${}^2R^4_{i,\gamma} \leftarrow \sum_{\delta \in A} \frac{1}{2} Z^*_{\delta,\gamma} \tau^9_{\delta,\gamma,i} \quad (2r_T^2 N_o) \quad (12018)$$

Raw expression

$${}^2R^4_{j,\zeta} \leftarrow - \sum_{\gamma \in A} \sum_{i \in O} \sum_{k \in O} \sum_{l \in O} \sum_{a \in V} \sum_{b \in V} \sum_{c \in V} {}^1T_{b,k} Y^{1,*}_{a,\gamma} Y^{2,*}_{i,\gamma} Z^*_{\gamma,\zeta} Y^{3,*}_{b,\zeta} {}^2D^{a,i,b,j} {}^2T_{c,l,a,i} V_{l,c,k,j} \quad (12007)$$

Raw expression

$${}^2R^4_{j,\zeta} \leftarrow - \sum_{\gamma \in A} \sum_{i \in O} \sum_{k \in O} \sum_{l \in O} \sum_{a \in V} \sum_{b \in V} \sum_{c \in V} {}^1T_{c,k} Y^{1,*}_{a,\gamma} Y^{2,*}_{i,\gamma} Z^*_{\gamma,\zeta} Y^{3,*}_{b,\zeta} {}^2D^{a,i,b,j} {}^2T_{a,i,b,l} V_{k,c,l,j} \quad (12019)$$

Factorized expression

$$\tau^0_{\gamma,\delta,w} = \sum_{a \in V} {}^2D^3_{a,w} Y^1_{a,\gamma} Y^{3,*}_{a,\delta} \quad (3r_D r_T^2 N_v) \quad (12008)$$

$$\tau^0_{\gamma,\delta,w} = \sum_{a \in V} {}^2D^3_{a,w} Y^3_{a,\gamma} Y^{3,*}_{a,\delta} \quad (3r_D r_T^2 N_v) \quad (12020)$$

$$\tau^1_{\gamma,\alpha,w} = \sum_{i \in O} {}^2D^2_{i,w} W^2_{i,\alpha} Y^{2,*}_{i,\gamma} \quad (3r_D r_T r_V N_o) \quad (12009)$$

$$\tau^1_{\gamma,\delta,w} = \sum_{a \in V} {}^2D^1_{a,w} Y^1_{a,\gamma} Y^{1,*}_{a,\delta} \quad (3r_D r_T^2 N_v) \quad (12021)$$

$$\tau^2_{\alpha,i} = \sum_{a \in V} {}^1T_{a,i} W^4_{a,\alpha} \quad (2r_V N_o N_v) \quad (12022)$$

$$\tau^3_{\alpha,\beta} = \sum_{i \in O} W^1_{i,\alpha} \tau^2_{\beta,i} \quad (2r_V^2 N_o) \quad (12035)$$

$$\tau^3_{\alpha,\beta} = \sum_{i \in O} W^1_{i,\alpha} \tau^2_{\beta,i} \quad (2r_V^2 N_o) \quad (12023)$$

$$\tau^4_{\alpha,i} = \sum_{\beta \in B} X_{\alpha,\beta} W^3_{i,\beta} \tau^3_{\alpha,\beta} \quad (3r_V^2 N_o) \quad (12036)$$

$$\tau^4_{\alpha,i} = \sum_{\beta \in B} X_{\alpha,\beta} W^3_{i,\beta} \tau^3_{\alpha,\beta} \quad (3r_V^2 N_o) \quad (12024)$$

$$\tau^5_{i,j} = \sum_{\alpha \in B} W^2_{i,\alpha} \tau^4_{\alpha,j} \quad (2r_V N_o^2) \quad (12037)$$

$$\tau^5_{i,j} = \sum_{\alpha \in B} W^2_{i,\alpha} \tau^4_{\alpha,j} \quad (2r_V N_o^2) \quad (12025)$$

$$\tau^6_{\gamma,i} = \sum_{j \in O} Y^4_{j,\gamma} \tau^5_{i,j} \quad (2r_T N_o^2) \quad (12038)$$

$$\tau^6_{\gamma,i} = \sum_{j \in O} Y^2_{j,\gamma} \tau^5_{i,j} \quad (2r_T N_o^2) \quad (12026)$$

$$\tau^7_{\gamma,\delta,w} = \sum_{i \in O} {}^2D^2_{i,w} Y^{2,*}_{i,\delta} \tau^6_{\gamma,i} \quad (3r_D r_T^2 N_o) \quad (12039)$$

$$\tau^7_{\gamma,\delta,w} = \sum_{i \in O} {}^2D^2_{i,w} Y^{2,*}_{i,\delta} \tau^6_{\gamma,i} \quad (3r_D r_T^2 N_o) \quad (12027)$$

$$\tau^8_{\gamma,\delta,w} = \sum_{\epsilon \in A} Z^*_{\epsilon,\delta} \tau^1_{\gamma,\epsilon,w} \tau^7_{\gamma,\epsilon,w} \quad (3r_D r_T^3) \quad (12040)$$

$$\tau^8_{\gamma,\delta,w} = \sum_{\epsilon \in A} Z^*_{\epsilon,\delta} \tau^1_{\gamma,\epsilon,w} \tau^7_{\gamma,\epsilon,w} \quad (3r_D r_T^3) \quad (12028)$$

$$\tau^9_{\gamma,\delta,w} = \sum_{\epsilon \in A} Z_{\gamma,\epsilon} \tau^8_{\epsilon,\delta,w} \quad (2r_D r_T^3) \quad (12041)$$

$$\tau^9_{\gamma,\delta,w} = \sum_{\epsilon \in A} Z_{\gamma,\epsilon} \tau^8_{\epsilon,\delta,w} \quad (2r_D r_T^3) \quad (12029)$$

$${}^2R^4_{i,\gamma} \leftarrow \sum_{\delta \in A} \sum_{w \in D} \frac{1}{2} {}^2D^4_{i,w} Y^2_{i,\delta} \tau^0_{\delta,\gamma,w} \tau^9_{\delta,\gamma,w} \quad (4r_D r_T^2 N_o) \quad (12042)$$

$${}^2R^4_{i,\gamma} \leftarrow \sum_{\delta \in A} \sum_{w \in D} \frac{1}{2} {}^2D^4_{i,w} Y^4_{i,\delta} \tau^0_{\delta,\gamma,w} \tau^9_{\delta,\gamma,w} \quad (4r_D r_T^2 N_o) \quad (12030)$$

Raw expression

$${}^2R^4_{j,\zeta} \leftarrow - \sum_{\gamma \in A} \sum_{i \in O} \sum_{k \in O} \sum_{l \in O} \sum_{a \in V} \sum_{b \in V} \sum_{c \in V} {}^1T_{c,k} Y^{1,*}_{a,\gamma} Y^{2,*}_{i,\gamma} Z^*_{\gamma,\zeta} Y^{3,*}_{b,\zeta} {}^2D^{a,i,b,j} {}^2T_{b,j,a,l} V_{l,i,k,c} \quad (12043)$$

Raw expression

$${}^2R^4_{j,\zeta} \leftarrow - \sum_{\gamma \in A} \sum_{i \in O} \sum_{k \in O} \sum_{l \in O} \sum_{a \in V} \sum_{b \in V} \sum_{c \in V} {}^1T_{c,k} Y^{1,*}_{a,\gamma} Y^{2,*}_{i,\gamma} Z^*_{\gamma,\zeta} Y^{3,*}_{b,\zeta} {}^2D^{a,i,b,j} {}^2T_{a,l,b,j} V_{l,i,k,c} \quad (12031)$$

Factorized expression

$$\tau^0_{\gamma,\delta,w} = \sum_{a \in V} {}^2D^3_{a,w} Y^3_{a,\gamma} Y^{3,*}_{a,\delta} \quad (3r_D r_T^2 N_v) \quad (12044)$$

Factorized expression

$$\tau^0_{\gamma,\delta,w} = \sum_{a \in V} {}^2D^3_{a,w} Y^1_{a,\gamma} Y^{3,*}_{a,\delta} \quad (3r_D r_T^2 N_v) \quad (12032)$$

$$\tau^1_{\gamma,\delta,w} = \sum_{a \in V} {}^2D^1_{a,w} Y^1_{a,\gamma} Y^{1,*}_{a,\delta} \quad (3r_D r_T^2 N_v) \quad (12045)$$

$$\tau^1_{\gamma,\delta,w} = \sum_{a \in V} {}^2D^1_{a,w} Y^3_{a,\gamma} Y^{1,*}_{a,\delta} \quad (3r_D r_T^2 N_v) \quad (12033)$$

$$\tau^2_{\gamma,\delta,w} = \sum_{i \in O} {}^2D^2_{i,w} Y^2_{i,\gamma} Y^{2,*}_{i,\delta} \quad (3r_D r_T^2 N_o) \quad (12046)$$

$$\tau^2_{\alpha,i} = \sum_{a \in V} {}^1T_{a,i} W^4_{a,\alpha} \quad (2r_V N_o N_v) \quad (12034)$$

$$\tau^3_{\gamma,\delta,w} = \sum_{\epsilon \in A} Z^*_{\epsilon,\delta} \tau^1_{\gamma,\epsilon,w} \tau^2_{\gamma,\epsilon,w} \quad (3r_D r_T^3) \quad (12047)$$

$$\tau_{\gamma,\delta,w}^4 = \sum_{\epsilon \in A} Z_{\epsilon,\gamma} \tau_{\epsilon,\delta,w}^3 \quad (2r_D r_T^3) \quad (12048)$$

$$\tau_{\alpha,i}^5 = \sum_{a \in V} {}^1T_{a,i} W_{a,\alpha}^2 \quad (2r_V N_o N_v) \quad (12049)$$

$$\tau_{\alpha,\beta}^6 = \sum_{i \in O} W_{i,\beta}^3 \tau_{\alpha,i}^5 \quad (2r_V^2 N_o) \quad (12050)$$

$$\tau_{\alpha,i}^7 = \sum_{\beta \in B} X_{\alpha,\beta} W_{i,\beta}^4 \tau_{\alpha,\beta}^6 \quad (3r_V^2 N_o) \quad (12051)$$

$$\tau_{i,j}^8 = \sum_{\alpha \in B} W_{i,\alpha}^1 \tau_{\alpha,j}^7 \quad (2r_V N_o^2) \quad (12052)$$

$$\tau_{\gamma,i}^9 = \sum_{j \in O} Y_{j,\gamma}^4 \tau_{j,i}^8 \quad (2r_T N_o^2) \quad (12053)$$

$${}^2R_{i,\gamma}^4 \leftarrow \sum_{\delta \in A} \sum_{w \in D} \frac{1}{2} {}^2D_{i,w}^4 \tau_{\delta,i}^9 \tau_{\delta,\gamma,w}^0 \tau_{\delta,\gamma,w}^4 \quad (4r_D r_T^2 N_o) \quad (12054)$$

Raw expression

$${}^2R_{j,\zeta}^4 \leftarrow - \sum_{\gamma \in A} \sum_{i \in O} \sum_{k \in O} \sum_{l \in O} \sum_{a \in V} \sum_{b \in V} \sum_{c \in V} {}^1T_{c,k} Y_{a,\gamma}^{1,*} Y_{i,\gamma}^{2,*} Z_{\gamma,\zeta}^* Y_{b,\zeta}^{3,*} {}^2D_{a,i,b,j} {}^2T_{b,l,a,i} V_{k,c,l,j} \quad (12055)$$

Factorized expression

$$\tau_{\gamma,\delta,w}^0 = \sum_{a \in V} {}^2D_{a,w}^3 Y_{a,\gamma}^1 Y_{a,\delta}^{3,*} \quad (3r_D r_T^2 N_v) \quad (12056)$$

$$\tau_{\gamma,\delta,w}^1 = \sum_{a \in V} {}^2D_{a,w}^1 Y_{a,\gamma}^3 Y_{a,\delta}^{1,*} \quad (3r_D r_T^2 N_v) \quad (12057)$$

$$\tau_{\gamma,\delta,w}^2 = \sum_{i \in O} {}^2D_{i,w}^2 Y_{i,\gamma}^4 Y_{i,\delta}^{2,*} \quad (3r_D r_T^2 N_o) \quad (12058)$$

$$\tau_{\gamma,\delta,w}^3 = \sum_{\epsilon \in A} Z_{\epsilon,\delta}^* \tau_{\gamma,\epsilon,w}^1 \tau_{\gamma,\epsilon,w}^2 \quad (3r_D r_T^3) \quad (12059)$$

$$\tau_{\gamma,\delta,w}^4 = \sum_{\epsilon \in A} Z_{\gamma,\epsilon} \tau_{\epsilon,\delta,w}^3 \quad (2r_D r_T^3) \quad (12060)$$

$$\tau_{\alpha,i}^5 = \sum_{a \in V} {}^1T_{a,i} W_{a,\alpha}^2 \quad (2r_V N_o N_v) \quad (12061)$$

$$\tau_{\alpha,\beta}^6 = \sum_{i \in O} W_{i,\beta}^3 \tau_{\alpha,i}^5 \quad (2r_V^2 N_o) \quad (12062)$$

$$\tau_{\alpha,i}^7 = \sum_{\beta \in B} X_{\alpha,\beta} W_{i,\beta}^4 \tau_{\alpha,\beta}^6 \quad (3r_V^2 N_o) \quad (12063)$$

$$\tau_{i,j}^8 = \sum_{\alpha \in B} W_{i,\alpha}^1 \tau_{\alpha,j}^7 \quad (2r_V N_o^2) \quad (12064)$$

$$\tau_{\gamma,i}^9 = \sum_{j \in O} Y_{j,\gamma}^2 \tau_{j,i}^8 \quad (2r_T N_o^2) \quad (12065)$$

$${}^2R_{i,\gamma}^4 \leftarrow \sum_{\delta \in A} \sum_{w \in D} \frac{1}{2} {}^2D_{i,w}^4 \tau_{\delta,i}^9 \tau_{\delta,\gamma,w}^0 \tau_{\delta,\gamma,w}^4 \quad (4r_D r_T^2 N_o) \quad (12066)$$

### G. Contributions from $(H^1 T^1 T^1 T^1 T)_c$

Raw expression

$${}^2R_{j,\zeta}^4 \leftarrow \sum_{\gamma \in A} \sum_{i \in O} \sum_{k \in O} \sum_{l \in O} \sum_{a \in V} \sum_{b \in V} \sum_{c \in V} \sum_{d \in V} {}^1T_{a,k} {}^1T_{b,l} {}^1T_{c,i} {}^1T_{d,j} Y_{a,\gamma}^{1,*} Y_{i,\gamma}^{2,*} Z_{\gamma,\zeta}^* Y_{b,\zeta}^{3,*} {}^2D_{a,i,b,j} V_{k,c,l,d} \quad (12067)$$

Factorized expression

$$\tau_{\gamma,w,i}^0 = \sum_{a \in V} {}^2D_{a,w}^3 {}^1T_{a,i} Y_{a,\gamma}^{3,*} \quad (3r_D r_T N_o N_v) \quad (12068)$$

$$\tau_{\gamma,\alpha,w}^1 = \sum_{i \in O} W_{i,\alpha}^3 \tau_{\gamma,w,i}^0 \quad (2r_D r_T r_V N_o) \quad (12069)$$

$$\tau_{\alpha,i}^2 = \sum_{a \in V} {}^1T_{a,i} W_{a,\alpha}^2 \quad (2r_V N_o N_v) \quad (12070)$$

$$\tau_{\gamma,\alpha,w}^3 = \sum_{i \in O} {}^2D_{i,w}^2 Y_{i,\gamma}^{2,*} \tau_{\alpha,i}^2 \quad (3r_D r_T r_V N_o) \quad (12071)$$

$$\tau_{\gamma,w,i}^4 = \sum_{a \in V} {}^2D_{a,w}^1 {}^1T_{a,i} Y_{a,\gamma}^{1,*} \quad (3r_D r_T N_o N_v) \quad (12072)$$

$$\tau_{\gamma,w,i}^3 = \sum_{a \in V} {}^2D_{a,w}^1 {}^1T_{a,i} Y_{a,\gamma}^{1,*} \quad (3r_D r_T N_o N_v) \quad (12083)$$

$$\tau_{\gamma,\alpha,w}^5 = \sum_{i \in O} W_{i,\alpha}^1 \tau_{\gamma,w,i}^4 \quad (2r_D r_T r_V N_o) \quad (12073)$$

$$\tau_{\gamma,\alpha,w}^4 = \sum_{i \in O} W_{i,\alpha}^1 \tau_{\gamma,w,i}^3 \quad (2r_D r_T r_V N_o) \quad (12084)$$

$$\tau_{\gamma,\alpha,w}^6 = \sum_{\beta \in B} X_{\beta,\alpha} \tau_{\gamma,\beta,w}^3 \tau_{\gamma,\beta,w}^5 \quad (3r_D r_T r_V^2) \quad (12074)$$

$$\tau_{\gamma,\alpha}^5 = \sum_{a \in V} W_{a,\alpha}^4 Y_{a,\gamma}^3 \quad (2r_T r_V N_v) \quad (12085)$$

$$\tau_{\gamma,\alpha,w}^7 = \sum_{\delta \in A} Z_{\delta,\gamma}^* \tau_{\delta,\alpha,w}^6 \quad (2r_D r_T^2 r_V) \quad (12075)$$

$$\tau_{\gamma,\alpha}^6 = \sum_{i \in O} W_{i,\alpha}^3 Y_{i,\gamma}^4 \quad (2r_T r_V N_o) \quad (12086)$$

$$\tau_{\alpha,i}^8 = \sum_{a \in V} {}^1T_{a,i} W_{a,\alpha}^4 \quad (2r_V N_o N_v) \quad (12076)$$

$$\tau_{\gamma,\alpha}^7 = \sum_{\beta \in B} X_{\alpha,\beta} \tau_{\gamma,\beta}^5 \tau_{\gamma,\beta}^6 \quad (3r_T r_V^2) \quad (12087)$$

$$\tau_{\gamma,w,i}^9 = \sum_{\alpha \in B} \tau_{\alpha,i}^8 \tau_{\gamma,\alpha,w}^1 \tau_{\gamma,\alpha,w}^7 \quad (3r_D r_T r_V N_o) \quad (12077)$$

$$\tau_{\gamma,\alpha}^8 = \sum_{\delta \in A} Z_{\gamma,\delta} \tau_{\delta,\alpha}^7 \quad (2r_T^2 r_V) \quad (12088)$$

$${}^2R_{i,\gamma}^4 \leftarrow \sum_{w \in D} {}^2D_{i,w}^4 \tau_{\gamma,w,i}^9 \quad (2r_D r_T N_o) \quad (12078)$$

$$\tau_{\gamma,\delta,w}^9 = \sum_{\alpha \in B} \tau_{\gamma,\alpha}^8 \tau_{\delta,\alpha,w}^2 \tau_{\delta,\alpha,w}^4 \quad (3r_D r_T^2 r_V) \quad (12089)$$

$$\tau_{\gamma,\delta,w}^{10} = \sum_{\epsilon \in A} Z_{\epsilon,\delta}^* \tau_{\gamma,\epsilon,w}^9 \quad (2r_D r_T^3) \quad (12090)$$

## H. Contributions from $(H^1 T^1 T^2 T)_c$

Raw expression

$${}^2R_{j,\zeta}^4 \leftarrow \sum_{\gamma \in A} \sum_{i \in O} \sum_{k \in O} \sum_{l \in O} \sum_{a \in V} \sum_{b \in V} \sum_{c \in V} \sum_{d \in V} \frac{1}{2} \quad (12079)$$

$${}^1T_{a,k} {}^1T_{b,l} Y_{a,\gamma}^{1,*} Y_{i,\gamma}^{2,*} Z_{\gamma,\zeta}^* Y_{b,\zeta}^{3,*} {}^2D_{a,i,b,j} {}^2T_{c,i,d,j} V_{k,c,l,d}$$

Factorized expression

$$\tau_{\gamma,\delta,w}^0 = \sum_{a \in V} {}^2D_{a,w}^3 Y_{a,\gamma}^1 Y_{a,\delta}^{3,*} \quad (3r_D r_T^2 N_v) \quad (12080)$$

$$\tau_{\alpha,i}^1 = \sum_{a \in V} {}^1T_{a,i} W_{a,\alpha}^2 \quad (2r_V N_o N_v) \quad (12081)$$

$$\tau_{\gamma,\alpha,w}^2 = \sum_{i \in O} {}^2D_{i,w}^2 Y_{i,\gamma}^{2,*} \tau_{\alpha,i}^1 \quad (3r_D r_T r_V N_o) \quad (12082)$$

$${}^2R_{i,\gamma}^4 \leftarrow - \sum_{\delta \in A} \sum_{w \in D} {}^2D_{i,w}^4 Y_{i,\delta}^2 \tau_{\delta,\gamma,w}^0 \tau_{\delta,\gamma,w}^{10} \quad (4r_D r_T^2 N_o) \quad (12091)$$

Raw expression

$${}^2R_{j,\zeta}^4 \leftarrow \sum_{\gamma \in A} \sum_{i \in O} \sum_{k \in O} \sum_{l \in O} \sum_{a \in V} \sum_{b \in V} \sum_{c \in V} \sum_{d \in V} \frac{1}{2} \quad (12092)$$

$${}^1T_{a,k} {}^1T_{b,l} Y_{a,\gamma}^{1,*} Y_{i,\gamma}^{2,*} Z_{\gamma,\zeta}^* Y_{b,\zeta}^{3,*} {}^2D_{a,i,b,j} {}^2T_{c,j,d,i} V_{k,d,l,c}$$

Factorized expression

$$\tau_{\gamma,\delta,w}^0 = \sum_{a \in V} {}^2D_{a,w}^3 Y_{a,\gamma}^3 Y_{a,\delta}^{3,*} \quad (3r_D r_T^2 N_v) \quad (12093)$$

$$\tau_{\alpha,i}^1 = \sum_{a \in V} {}^1T_{a,i} W_{a,\alpha}^2 \quad (2r_V N_o N_v) \quad (12094)$$

$$\tau^2_{\gamma,\alpha,w} = \sum_{i \in O} {}^2D^2_{i,w} Y^{2,*}_{i,\gamma} \tau^1_{\alpha,i} \quad (3r_D r_T r_V N_o) \quad (12095)$$

$$\tau^3_{\gamma,w,i} = \sum_{a \in V} {}^2D^1_{a,w} {}^1T_{a,i} Y^{1,*}_{a,\gamma} \quad (3r_D r_T N_o N_v) \quad (12096)$$

$$\tau^4_{\gamma,\alpha,w} = \sum_{i \in O} W^1_{i,\alpha} \tau^3_{\gamma,w,i} \quad (2r_D r_T r_V N_o) \quad (12097)$$

$$\tau^5_{\gamma,\alpha} = \sum_{a \in V} W^4_{a,\alpha} Y^1_{a,\gamma} \quad (2r_T r_V N_v) \quad (12098)$$

$$\tau^6_{\gamma,\alpha} = \sum_{i \in O} W^3_{i,\alpha} Y^2_{i,\gamma} \quad (2r_T r_V N_o) \quad (12099)$$

$$\tau^7_{\gamma,\alpha} = \sum_{\beta \in B} X_{\alpha,\beta} \tau^5_{\gamma,\beta} \tau^6_{\gamma,\beta} \quad (3r_T r_V^2) \quad (12100)$$

$$\tau^8_{\gamma,\alpha} = \sum_{\delta \in A} Z_{\delta,\gamma} \tau^7_{\delta,\alpha} \quad (2r_T^2 r_V) \quad (12101)$$

$$\tau^9_{\gamma,\delta,w} = \sum_{\alpha \in B} \tau^8_{\gamma,\alpha} \tau^2_{\delta,\alpha,w} \tau^4_{\delta,\alpha,w} \quad (3r_D r_T^2 r_V) \quad (12102)$$

$$\tau^{10}_{\gamma,\delta,w} = \sum_{\epsilon \in A} Z^*_{\epsilon,\delta} \tau^9_{\gamma,\epsilon,w} \quad (2r_D r_T^3) \quad (12103)$$

$${}^2R^4_{i,\gamma} \leftarrow - \sum_{\delta \in A} \sum_{w \in D} {}^2D^4_{i,w} Y^4_{i,\delta} \tau^0_{\delta,\gamma,w} \tau^{10}_{\delta,\gamma,w} \quad (4r_D r_T^2 N_o)^2 \quad (12104)$$

Raw expression

$${}^2R^4_{j,\zeta} \leftarrow \sum_{\gamma \in A} \sum_{i \in O} \sum_{k \in O} \sum_{l \in O} \sum_{a \in V} \sum_{b \in V} \sum_{c \in V} \sum_{d \in V} \frac{1}{2} \quad (12105)$$

$${}^1T_{a,k} {}^1T_{c,i} Y^{1,*}_{a,\gamma} Y^{2,*}_{i,\gamma} Z^*_{\gamma,\zeta} Y^{3,*}_{b,\zeta} {}^2D^{a,i,b,j} {}^2T_{b,j,d,l} V_{k,d,l,c}$$

Factorized expression

$$\tau^0_{\gamma,\delta,w} = \sum_{a \in V} {}^2D^3_{a,w} Y^1_{a,\gamma} Y^{3,*}_{a,\delta} \quad (3r_D r_T^2 N_v) \quad (12106)$$

$$\tau^1_{\gamma,\delta,w} = \sum_{i \in O} {}^2D^2_{i,w} Y^4_{i,\gamma} Y^{2,*}_{i,\delta} \quad (3r_D r_T^2 N_o) \quad (12107)$$

$$\tau^2_{\gamma,w,i} = \sum_{a \in V} {}^2D^1_{a,w} {}^1T_{a,i} Y^{1,*}_{a,\gamma} \quad (3r_D r_T N_o N_v) \quad (12108)$$

$$\tau^3_{\alpha,i} = \sum_{a \in V} {}^1T_{a,i} W^4_{a,\alpha} \quad (2r_V N_o N_v) \quad (12109)$$

$$\tau^4_{\alpha} = \sum_{i \in O} W^3_{i,\alpha} \tau^3_{\alpha,i} \quad (2r_V N_o) \quad (12110)$$

$$\tau^5_{\alpha} = \sum_{\beta \in B} \tau^4_{\beta} X_{\alpha,\beta} \quad (2r_V^2) \quad (12111)$$

$$\tau^6_{i,a} = \sum_{\alpha \in B} \tau^5_{\alpha} W^1_{i,\alpha} W^2_{a,\alpha} \quad (3r_V N_o N_v) \quad (12112)$$

$$\tau^7_{\gamma,i} = \sum_{a \in V} Y^3_{a,\gamma} \tau^6_{i,a} \quad (2r_T N_o N_v) \quad (12113)$$

$$\tau^8_{\gamma,\delta,w} = \sum_{i \in O} \tau^7_{\gamma,i} \tau^2_{\delta,w,i} \quad (2r_D r_T^2 N_o) \quad (12114)$$

$$\tau^9_{\gamma,\delta,w} = \sum_{\epsilon \in A} Z^*_{\epsilon,\delta} \tau^1_{\gamma,\epsilon,w} \tau^8_{\gamma,\epsilon,w} \quad (3r_D r_T^3) \quad (12115)$$

$$\tau^{10}_{\gamma,\delta,w} = \sum_{\epsilon \in A} Z_{\gamma,\epsilon} \tau^9_{\epsilon,\delta,w} \quad (2r_D r_T^3) \quad (12116)$$

$${}^2R^4_{i,\gamma} \leftarrow - \sum_{\delta \in A} \sum_{w \in D} {}^2D^4_{i,w} Y^2_{i,\delta} \tau^0_{\delta,\gamma,w} \tau^{10}_{\delta,\gamma,w} \quad (4r_D r_T^2 N_o) \quad (12117)$$

Raw expression

$${}^2R^4_{j,\zeta} \leftarrow \sum_{\gamma \in A} \sum_{i \in O} \sum_{k \in O} \sum_{l \in O} \sum_{a \in V} \sum_{b \in V} \sum_{c \in V} \sum_{d \in V} \frac{1}{2} \quad (12118)$$

$${}^1T_{a,k} {}^1T_{c,i} Y^{1,*}_{a,\gamma} Y^{2,*}_{i,\gamma} Z^*_{\gamma,\zeta} Y^{3,*}_{b,\zeta} {}^2D^{a,i,b,j} {}^2T_{b,l,d,j} V_{k,c,l,d}$$

Factorized expression

$$\tau^0_{\gamma,\delta,w} = \sum_{a \in V} {}^2D^3_{a,w} Y^3_{a,\gamma} Y^{3,*}_{a,\delta} \quad (3r_D r_T^2 N_v) \quad (12119)$$

$$\tau^1_{\gamma,\delta,w} = \sum_{i \in O} {}^2D^2_{i,w} Y^2_{i,\gamma} Y^{2,*}_{i,\delta} \quad (3r_D r_T^2 N_o) \quad (12120)$$

$$\tau^1_{\gamma,\alpha,w} = \sum_{i \in O} W^1_{i,\alpha} \tau^0_{\gamma,w,i} \quad (2r_D r_T r_V N_o) \quad (12133)$$

$$\tau^2_{\gamma,w,i} = \sum_{a \in V} {}^2D^1_{a,w} {}^1T_{a,i} Y^{1,*}_{a,\gamma} \quad (3r_D r_T N_o N_v) \quad (12121)$$

$$\tau^2_{\gamma,\alpha} = \sum_{a \in V} W^4_{a,\alpha} Y^3_{a,\gamma} \quad (2r_T r_V N_v) \quad (12134)$$

$$\tau^3_{\alpha,i} = \sum_{a \in V} {}^1T_{a,i} W^4_{a,\alpha} \quad (2r_V N_o N_v) \quad (12122)$$

$$\tau^3_{\gamma,\alpha} = \sum_{i \in O} W^3_{i,\alpha} Y^4_{i,\gamma} \quad (2r_T r_V N_o) \quad (12135)$$

$$\tau^4_{\alpha} = \sum_{i \in O} W^3_{i,\alpha} \tau^3_{\alpha,i} \quad (2r_V N_o) \quad (12123)$$

$$\tau^4_{\gamma,\alpha} = \sum_{\beta \in B} X_{\alpha,\beta} \tau^2_{\gamma,\beta} \tau^3_{\gamma,\beta} \quad (3r_T r_V^2) \quad (12136)$$

$$\tau^5_{\alpha} = \sum_{\beta \in B} \tau^4_{\beta} X_{\alpha,\beta} \quad (2r_V^2) \quad (12124)$$

$$\tau^5_{\gamma,\alpha} = \sum_{\delta \in A} Z_{\gamma,\delta} \tau^4_{\delta,\alpha} \quad (2r_T^2 r_V) \quad (12137)$$

$$\tau^6_{i,a} = \sum_{\alpha \in B} \tau^5_{\alpha} W^1_{i,\alpha} W^2_{a,\alpha} \quad (3r_V N_o N_v) \quad (12125)$$

$$\tau^6_{\gamma,\delta,w} = \sum_{a \in V} {}^2D^1_{a,w} Y^1_{a,\gamma} Y^{1,*}_{a,\delta} \quad (3r_D r_T^2 N_v) \quad (12138)$$

$$\tau^7_{\gamma,i} = \sum_{a \in V} Y^1_{a,\gamma} \tau^6_{i,a} \quad (2r_T N_o N_v) \quad (12126)$$

$$\tau^7_{\gamma,\delta,w} = \sum_{i \in O} {}^2D^2_{i,w} Y^2_{i,\gamma} Y^{2,*}_{i,\delta} \quad (3r_D r_T^2 N_o) \quad (12139)$$

$$\tau^8_{\gamma,\delta,w} = \sum_{i \in O} \tau^7_{\gamma,i} \tau^2_{\delta,w,i} \quad (2r_D r_T^2 N_o) \quad (12127)$$

$$\tau^8_{\gamma,\delta,w} = \sum_{\epsilon \in A} Z^*_{\epsilon,\delta} \tau^6_{\gamma,\epsilon,w} \tau^7_{\gamma,\epsilon,w} \quad (3r_D r_T^3) \quad (12140)$$

$$\tau^9_{\gamma,\delta,w} = \sum_{\epsilon \in A} Z^*_{\epsilon,\delta} \tau^1_{\gamma,\epsilon,w} \tau^8_{\gamma,\epsilon,w} \quad (3r_D r_T^3) \quad (12128)$$

$$\tau^9_{\gamma,\alpha,w} = \sum_{\delta \in A} \tau^5_{\delta,\alpha} \tau^8_{\delta,\gamma,w} \quad (2r_D r_T^2 r_V) \quad (12141)$$

$$\tau^{10}_{\gamma,\delta,w} = \sum_{\epsilon \in A} Z_{\epsilon,\gamma} \tau^9_{\epsilon,\delta,w} \quad (2r_D r_T^3) \quad (12129)$$

$$\tau^{10}_{\alpha,i} = \sum_{a \in V} {}^1T_{a,i} W^2_{a,\alpha} \quad (2r_V N_o N_v) \quad (12142)$$

$${}^2R^4_{i,\gamma} \leftarrow - \sum_{\delta \in A} \sum_{w \in D} {}^2D^4_{i,w} Y^4_{i,\delta} \tau^0_{\delta,\gamma,w} \tau^{10}_{\delta,\gamma,w} \quad (4r_D r_T^2 N_o) \quad (12130)$$

$$\tau^{11}_{\gamma,w,i} = \sum_{\alpha \in B} \tau^{10}_{\alpha,i} \tau^1_{\gamma,\alpha,w} \tau^9_{\gamma,\alpha,w} \quad (3r_D r_T r_V N_o) \quad (12143)$$

Raw expression

$${}^2R^4_{j,\zeta} \leftarrow \sum_{\gamma \in A} \sum_{i \in O} \sum_{k \in O} \sum_{l \in O} \sum_{a \in V} \sum_{b \in V} \sum_{c \in V} \sum_{d \in V} \frac{1}{2} \quad (12131)$$

$${}^1T_{a,k} {}^1T_{c,i} Y^{1,*}_{a,\gamma} Y^{2,*}_{i,\gamma} Z^*_{\gamma,\zeta} Y^{3,*}_{b,\zeta} {}^2D^{a,i,b,j} {}^2T_{d,j,b,l} V_{k,c,l,d}$$

Factorized expression

$$\tau^0_{\gamma,w,i} = \sum_{a \in V} {}^2D^3_{a,w} {}^1T_{a,i} Y^{3,*}_{a,\gamma} \quad (3r_D r_T N_o N_v) \quad (12132)$$

$${}^2R^4_{i,\gamma} \leftarrow - \sum_{w \in D} {}^2D^4_{i,w} \tau^{11}_{\gamma,w,i} \quad (2r_D r_T N_o) \quad (12144)$$

Raw expression

$${}^2R^4_{j,\zeta} \leftarrow \sum_{\gamma \in A} \sum_{i \in O} \sum_{k \in O} \sum_{l \in O} \sum_{a \in V} \sum_{b \in V} \sum_{c \in V} \sum_{d \in V} \frac{1}{2} \quad (12145)$$

$${}^1T_{a,k} {}^1T_{c,i} Y^{1,*}_{a,\gamma} Y^{2,*}_{i,\gamma} Z^*_{\gamma,\zeta} Y^{3,*}_{b,\zeta} {}^2D^{a,i,b,j} {}^2T_{d,l,b,j} V_{k,d,l,c}$$

Factorized expression

$$\tau_{\gamma,w,i}^0 = \sum_{a \in V} {}^2D_{a,w}^3 {}^1T_{a,i} Y_{a,\gamma}^{3,*} \quad (3r_D r_T N_o N_v) \quad (12146)$$

$$\tau_{\gamma,\alpha,w}^1 = \sum_{i \in O} W_{i,\alpha}^1 \tau_{\gamma,w,i}^0 \quad (2r_D r_T r_V N_o) \quad (12147)$$

$$\tau_{\gamma,\delta,w}^2 = \sum_{a \in V} {}^2D_{a,w}^1 Y_{a,\gamma}^3 Y_{a,\delta}^{1,*} \quad (3r_D r_T^2 N_v) \quad (12148)$$

$$\tau_{\gamma,\delta,w}^3 = \sum_{i \in O} {}^2D_{i,w}^2 Y_{i,\gamma}^4 Y_{i,\delta}^{2,*} \quad (3r_D r_T^2 N_o) \quad (12149)$$

$$\tau_{\gamma,\delta,w}^4 = \sum_{\epsilon \in A} Z_{\epsilon,\delta}^* \tau_{\gamma,\epsilon,w}^2 \tau_{\gamma,\epsilon,w}^3 \quad (3r_D r_T^3) \quad (12150)$$

$$\tau_{\gamma,\alpha}^5 = \sum_{a \in V} W_{a,\alpha}^4 Y_{a,\gamma}^1 \quad (2r_T r_V N_v) \quad (12151)$$

$$\tau_{\gamma,\alpha}^6 = \sum_{i \in O} W_{i,\alpha}^3 Y_{i,\gamma}^2 \quad (2r_T r_V N_o) \quad (12152)$$

$$\tau_{\gamma,\alpha}^7 = \sum_{\beta \in B} X_{\alpha,\beta} \tau_{\gamma,\beta}^5 \tau_{\gamma,\beta}^6 \quad (3r_T r_V^2) \quad (12153)$$

$$\tau_{\gamma,\alpha}^8 = \sum_{\delta \in A} Z_{\delta,\gamma} \tau_{\delta,\alpha}^7 \quad (2r_T^2 r_V) \quad (12154)$$

$$\tau_{\gamma,\alpha,w}^9 = \sum_{\delta \in A} \tau_{\delta,\alpha}^8 \tau_{\delta,\gamma,w}^4 \quad (2r_D r_T^2 r_V) \quad (12155)$$

$$\tau_{\alpha,i}^{10} = \sum_{a \in V} {}^1T_{a,i} W_{a,\alpha}^2 \quad (2r_V N_o N_v) \quad (12156)$$

$$\tau_{\gamma,w,i}^{11} = \sum_{\alpha \in B} \tau_{\alpha,i}^{10} \tau_{\gamma,\alpha,w}^1 \tau_{\gamma,\alpha,w}^9 \quad (3r_D r_T r_V N_o) \quad (12157)$$

$${}^2R_{i,\gamma}^4 \leftarrow - \sum_{w \in D} {}^2D_{i,w}^4 \tau_{\gamma,w,i}^{11} \quad (2r_D r_T N_o) \quad (12158)$$

Raw expression

$${}^2R_{j,\zeta}^4 \leftarrow \sum_{\gamma \in A} \sum_{i \in O} \sum_{k \in O} \sum_{l \in O} \sum_{a \in V} \sum_{b \in V} \sum_{c \in V} \sum_{d \in V} \frac{1}{2} \quad (12159)$$

$${}^1T_{a,k} {}^1T_{c,j} Y_{a,\gamma}^{1,*} Y_{i,\gamma}^{2,*} Z_{\gamma,\zeta}^* Y_{b,\zeta}^{3,*} {}^2D_{a,i,b,j} {}^2T_{b,l,d,i} V_{k,d,l,c}$$

Factorized expression

$$\tau_{\gamma,w,i}^0 = \sum_{a \in V} {}^2D_{a,w}^3 {}^1T_{a,i} Y_{a,\gamma}^{3,*} \quad (3r_D r_T N_o N_v) \quad (12160)$$

$$\tau_{\alpha,i}^1 = \sum_{a \in V} {}^1T_{a,i} W_{a,\alpha}^4 \quad (2r_V N_o N_v) \quad (12161)$$

$$\tau_{\alpha}^2 = \sum_{i \in O} W_{i,\alpha}^3 \tau_{\alpha,i}^1 \quad (2r_V N_o) \quad (12162)$$

$$\tau_{\alpha}^3 = \sum_{\beta \in B} \tau_{\beta}^2 X_{\alpha,\beta} \quad (2r_V^2) \quad (12163)$$

$$\tau_{i,a}^4 = \sum_{\alpha \in B} \tau_{\alpha}^3 W_{i,\alpha}^1 W_{a,\alpha}^2 \quad (3r_V N_o N_v) \quad (12164)$$

$$\tau_{\gamma,i}^5 = \sum_{a \in V} Y_{a,\gamma}^3 \tau_{i,a}^4 \quad (2r_T N_o N_v) \quad (12165)$$

$$\tau_{\gamma,\delta,w}^6 = \sum_{i \in O} \tau_{\gamma,i}^5 \tau_{\delta,w,i}^0 \quad (2r_D r_T^2 N_o) \quad (12166)$$

$$\tau_{\gamma,\delta,w}^7 = \sum_{a \in V} {}^2D_{a,w}^1 Y_{a,\gamma}^1 Y_{a,\delta}^{1,*} \quad (3r_D r_T^2 N_v) \quad (12167)$$

$$\tau_{\gamma,\delta,w}^8 = \sum_{i \in O} {}^2D_{i,w}^2 Y_{i,\gamma}^2 Y_{i,\delta}^{2,*} \quad (3r_D r_T^2 N_o) \quad (12168)$$

$$\tau_{\gamma,\delta,w}^9 = \sum_{\epsilon \in A} Z_{\epsilon,\delta}^* \tau_{\gamma,\epsilon,w}^7 \tau_{\gamma,\epsilon,w}^8 \quad (3r_D r_T^3) \quad (12169)$$

$$\tau_{\gamma,\delta,w}^{10} = \sum_{\epsilon \in A} Z_{\epsilon,\gamma} \tau_{\epsilon,\delta,w}^9 \quad (2r_D r_T^3) \quad (12170)$$

$${}^2R_{i,\gamma}^4 \leftarrow - \sum_{\delta \in A} \sum_{w \in D} {}^2D_{i,w}^4 Y_{i,\delta}^4 \tau_{\delta,\gamma,w}^{10} \tau_{\delta,\gamma,w}^6 \quad (4r_D r_T^2 N_o) \quad (12171)$$



Raw expression

$${}^2R^4_{j,\zeta} \leftarrow \sum_{\gamma \in A} \sum_{i \in O} \sum_{k \in O} \sum_{l \in O} \sum_{a \in V} \sum_{b \in V} \sum_{c \in V} \sum_{d \in V} \frac{1}{2} \quad (12172)$$

$${}^1T_{a,k} \quad {}^1T_{c,j} \quad Y^{1,*}_{a,\gamma} \quad Y^{2,*}_{i,\gamma} \quad Z^*_{\gamma,\zeta}$$

$$Y^{3,*}_{b,\zeta} \quad {}^2D^{a,i,b,j} \quad {}^2T_{d,i,b,l} \quad V_{k,d,l,c}$$

Factorized expression

$$\tau^0_{\gamma,w,i} = \sum_{a \in V} {}^2D^3_{a,w} {}^1T_{a,i} Y^{3,*}_{a,\gamma} \quad (3r_D r_T N_o N_v) \quad (12173)$$

$$\tau^1_{\alpha,i} = \sum_{a \in V} {}^1T_{a,i} W^4_{a,\alpha} \quad (2r_V N_o N_v) \quad (12174)$$

$$\tau^2_{\alpha} = \sum_{i \in O} W^3_{i,\alpha} \tau^1_{\alpha,i} \quad (2r_V N_o) \quad (12175)$$

$$\tau^3_{\alpha} = \sum_{\beta \in B} \tau^2_{\beta} X_{\alpha,\beta} \quad (2r_V^2) \quad (12176)$$

$$\tau^4_{i,a} = \sum_{\alpha \in B} \tau^3_{\alpha} W^1_{i,\alpha} W^2_{a,\alpha} \quad (3r_V N_o N_v) \quad (12177)$$

$$\tau^5_{\gamma,i} = \sum_{a \in V} Y^1_{a,\gamma} \tau^4_{i,a} \quad (2r_T N_o N_v) \quad (12178)$$

$$\tau^6_{\gamma,\delta,w} = \sum_{i \in O} \tau^5_{\gamma,i} \tau^0_{\delta,w,i} \quad (2r_D r_T^2 N_o) \quad (12179)$$

$$\tau^7_{\gamma,\delta,w} = \sum_{a \in V} {}^2D^1_{a,w} Y^3_{a,\gamma} Y^{1,*}_{a,\delta} \quad (3r_D r_T^2 N_v) \quad (12180)$$

$$\tau^8_{\gamma,\delta,w} = \sum_{i \in O} {}^2D^2_{i,w} Y^4_{i,\gamma} Y^{2,*}_{i,\delta} \quad (3r_D r_T^2 N_o) \quad (12181)$$

$$\tau^9_{\gamma,\delta,w} = \sum_{\epsilon \in A} Z^*_{\epsilon,\delta} \tau^7_{\gamma,\epsilon,w} \tau^8_{\gamma,\epsilon,w} \quad (3r_D r_T^3) \quad (12182)$$

$$\tau^{10}_{\gamma,\delta,w} = \sum_{\epsilon \in A} Z_{\gamma,\epsilon} \tau^9_{\epsilon,\delta,w} \quad (2r_D r_T^3) \quad (12183)$$

$${}^2R^4_{i,\gamma} \leftarrow - \sum_{\delta \in A} \sum_{w \in D} {}^2D^4_{i,w} Y^2_{i,\delta} \tau^{10}_{\delta,\gamma,w} \tau^6_{\delta,\gamma,w} \quad (4r_D r_T^2 N_o)^2 R^4_{i,\gamma} \leftarrow - \sum_{\delta \in A} \sum_{w \in D} {}^2D^4_{i,w} Y^4_{i,\delta} \tau^0_{\delta,\gamma,w} \tau^{10}_{\delta,\gamma,w} \quad (4r_D r_T^2 N_o) \quad (12184)$$

Raw expression

$${}^2R^4_{j,\zeta} \leftarrow \sum_{\gamma \in A} \sum_{i \in O} \sum_{k \in O} \sum_{l \in O} \sum_{a \in V} \sum_{b \in V} \sum_{c \in V} \sum_{d \in V} \frac{1}{2} \quad (12185)$$

$${}^1T_{a,k} \quad {}^1T_{c,l} \quad Y^{1,*}_{a,\gamma} \quad Y^{2,*}_{i,\gamma} \quad Z^*_{\gamma,\zeta}$$

$$Y^{3,*}_{b,\zeta} \quad {}^2D^{a,i,b,j} \quad {}^2T_{b,j,d,i} \quad V_{k,c,l,d}$$

Factorized expression

$$\tau^0_{\gamma,\delta,w} = \sum_{a \in V} {}^2D^3_{a,w} Y^3_{a,\gamma} Y^{3,*}_{a,\delta} \quad (3r_D r_T^2 N_v) \quad (12186)$$

$$\tau^1_{\gamma,\delta,w} = \sum_{a \in V} {}^2D^1_{a,w} Y^1_{a,\gamma} Y^{1,*}_{a,\delta} \quad (3r_D r_T^2 N_v) \quad (12187)$$

$$\tau^2_{\alpha,i} = \sum_{a \in V} {}^1T_{a,i} W^2_{a,\alpha} \quad (2r_V N_o N_v) \quad (12188)$$

$$\tau^3_{\alpha} = \sum_{i \in O} W^1_{i,\alpha} \tau^2_{\alpha,i} \quad (2r_V N_o) \quad (12189)$$

$$\tau^4_{\alpha} = \sum_{\beta \in B} \tau^3_{\beta} X_{\beta,\alpha} \quad (2r_V^2) \quad (12190)$$

$$\tau^5_{i,a} = \sum_{\alpha \in B} \tau^4_{\alpha} W^3_{i,\alpha} W^4_{a,\alpha} \quad (3r_V N_o N_v) \quad (12191)$$

$$\tau^6_{i,j} = \sum_{a \in V} {}^1T_{a,i} \tau^5_{j,a} \quad (2N_o^2 N_v) \quad (12192)$$

$$\tau^7_{\gamma,i} = \sum_{j \in O} Y^2_{j,\gamma} \tau^6_{i,j} \quad (2r_T N_o^2) \quad (12193)$$

$$\tau^8_{\gamma,\delta,w} = \sum_{i \in O} {}^2D^2_{i,w} Y^{2,*}_{i,\delta} \tau^7_{\gamma,i} \quad (3r_D r_T^2 N_o) \quad (12194)$$

$$\tau^9_{\gamma,\delta,w} = \sum_{\epsilon \in A} Z^*_{\epsilon,\delta} \tau^1_{\gamma,\epsilon,w} \tau^8_{\gamma,\epsilon,w} \quad (3r_D r_T^3) \quad (12195)$$

$$\tau^{10}_{\gamma,\delta,w} = \sum_{\epsilon \in A} Z_{\epsilon,\gamma} \tau^9_{\epsilon,\delta,w} \quad (2r_D r_T^3) \quad (12196)$$

$${}^2R^4_{i,\gamma} \leftarrow - \sum_{\delta \in A} \sum_{w \in D} {}^2D^4_{i,w} Y^4_{i,\delta} \tau^0_{\delta,\gamma,w} \tau^{10}_{\delta,\gamma,w} \quad (4r_D r_T^2 N_o) \quad (12197)$$

Raw expression

$${}^2R^4_{j,\zeta} \leftarrow \sum_{\gamma \in A} \sum_{i \in O} \sum_{k \in O} \sum_{l \in O} \sum_{a \in V} \sum_{b \in V} \sum_{c \in V} \sum_{d \in V} \frac{1}{2} \quad (12198)$$

$${}^1T_{a,k} {}^1T_{c,l} Y^{1,*}_{a,\gamma} Y^{2,*}_{i,\gamma} Z^*_{\gamma,\zeta}$$

$$Y^{3,*}_{b,\zeta} {}^2D^{a,i,b,j} {}^2T_{d,i,b,j} V_{k,c,l,d}$$

Factorized expression

$$\tau^0_{\gamma,\delta,w} = \sum_{a \in V} {}^2D^3_{a,w} Y^1_{a,\gamma} Y^{3,*}_{a,\delta} \quad (3r_D r_T^2 N_v) \quad (12199)$$

$$\tau^1_{\gamma,\delta,w} = \sum_{a \in V} {}^2D^1_{a,w} Y^3_{a,\gamma} Y^{1,*}_{a,\delta} \quad (3r_D r_T^2 N_v) \quad (12200)$$

$$\tau^2_{\alpha,i} = \sum_{a \in V} {}^1T_{a,i} W^2_{a,\alpha} \quad (2r_V N_o N_v) \quad (12201)$$

$$\tau^3_{\alpha} = \sum_{i \in O} W^1_{i,\alpha} \tau^2_{\alpha,i} \quad (2r_V N_o) \quad (12202)$$

$$\tau^4_{\alpha} = \sum_{\beta \in B} \tau^3_{\beta} X_{\beta,\alpha} \quad (2r_V^2) \quad (12203)$$

$$\tau^5_{i,a} = \sum_{\alpha \in B} \tau^4_{\alpha} W^3_{i,\alpha} W^4_{a,\alpha} \quad (3r_V N_o N_v) \quad (12204)$$

$$\tau^6_{i,j} = \sum_{a \in V} {}^1T_{a,i} \tau^5_{j,a} \quad (2N_o^2 N_v) \quad (12205)$$

$$\tau^7_{\gamma,i} = \sum_{j \in O} Y^4_{j,\gamma} \tau^6_{i,j} \quad (2r_T N_o^2) \quad (12206)$$

$$\tau^8_{\gamma,\delta,w} = \sum_{i \in O} {}^2D^2_{i,w} Y^{2,*}_{i,\delta} \tau^7_{\gamma,i} \quad (3r_D r_T^2 N_o) \quad (12207)$$

$$\tau^9_{\gamma,\delta,w} = \sum_{\epsilon \in A} Z^*_{\epsilon,\delta} \tau^1_{\gamma,\epsilon,w} \tau^8_{\gamma,\epsilon,w} \quad (3r_D r_T^3) \quad (12208)$$

$$\tau^{10}_{\gamma,\delta,w} = \sum_{\epsilon \in A} Z_{\gamma,\epsilon} \tau^9_{\epsilon,\delta,w} \quad (2r_D r_T^3) \quad (12209)$$

$${}^2R^4_{i,\gamma} \leftarrow - \sum_{\delta \in A} \sum_{w \in D} {}^2D^4_{i,w} Y^2_{i,\delta} \tau^0_{\delta,\gamma,w} \tau^{10}_{\delta,\gamma,w} \quad (4r_D r_T^2 N_o)^2 R^4_{i,\gamma} \leftarrow - \sum_{\delta \in A} \sum_{w \in D} {}^2D^4_{i,w} \tau^{10}_{\delta,i} \tau^0_{\delta,\gamma,w} \tau^4_{\delta,\gamma,w} \quad (4r_D r_T^2 N_o) \quad (12210)$$

Raw expression

$${}^2R^4_{j,\zeta} \leftarrow \sum_{\gamma \in A} \sum_{i \in O} \sum_{k \in O} \sum_{l \in O} \sum_{a \in V} \sum_{b \in V} \sum_{c \in V} \sum_{d \in V} \frac{1}{2} \quad (12211)$$

$${}^1T_{b,k} {}^1T_{c,i} Y^{1,*}_{a,\gamma} Y^{2,*}_{i,\gamma} Z^*_{\gamma,\zeta}$$

$$Y^{3,*}_{b,\zeta} {}^2D^{a,i,b,j} {}^2T_{a,l,d,j} V_{k,d,l,c}$$

Factorized expression

$$\tau^0_{\gamma,\delta,w} = \sum_{a \in V} {}^2D^3_{a,w} Y^3_{a,\gamma} Y^{3,*}_{a,\delta} \quad (3r_D r_T^2 N_v) \quad (12212)$$

$$\tau^1_{\gamma,\delta,w} = \sum_{a \in V} {}^2D^1_{a,w} Y^1_{a,\gamma} Y^{1,*}_{a,\delta} \quad (3r_D r_T^2 N_v) \quad (12213)$$

$$\tau^2_{\gamma,\delta,w} = \sum_{i \in O} {}^2D^2_{i,w} Y^2_{i,\gamma} Y^{2,*}_{i,\delta} \quad (3r_D r_T^2 N_o) \quad (12214)$$

$$\tau^3_{\gamma,\delta,w} = \sum_{\epsilon \in A} Z^*_{\epsilon,\delta} \tau^1_{\gamma,\epsilon,w} \tau^2_{\gamma,\epsilon,w} \quad (3r_D r_T^3) \quad (12215)$$

$$\tau^4_{\gamma,\delta,w} = \sum_{\epsilon \in A} Z_{\epsilon,\gamma} \tau^3_{\epsilon,\delta,w} \quad (2r_D r_T^3) \quad (12216)$$

$$\tau^5_{\alpha,i} = \sum_{a \in V} {}^1T_{a,i} W^2_{a,\alpha} \quad (2r_V N_o N_v) \quad (12217)$$

$$\tau^6_{\alpha} = \sum_{i \in O} W^1_{i,\alpha} \tau^5_{\alpha,i} \quad (2r_V N_o) \quad (12218)$$

$$\tau^7_{\alpha} = \sum_{\beta \in B} \tau^6_{\beta} X_{\beta,\alpha} \quad (2r_V^2) \quad (12219)$$

$$\tau^8_{i,a} = \sum_{\alpha \in B} \tau^7_{\alpha} W^3_{i,\alpha} W^4_{a,\alpha} \quad (3r_V N_o N_v) \quad (12220)$$

$$\tau^9_{i,j} = \sum_{a \in V} {}^1T_{a,i} \tau^8_{j,a} \quad (2N_o^2 N_v) \quad (12221)$$

$$\tau^{10}_{\gamma,i} = \sum_{j \in O} Y^4_{j,\gamma} \tau^9_{i,j} \quad (2r_T N_o^2) \quad (12222)$$

$${}^2R^4_{i,\gamma} \leftarrow - \sum_{\delta \in A} \sum_{w \in D} {}^2D^4_{i,w} \tau^{10}_{\delta,i} \tau^0_{\delta,\gamma,w} \tau^4_{\delta,\gamma,w} \quad (4r_D r_T^2 N_o)^2 R^4_{i,\gamma} \leftarrow - \sum_{\delta \in A} \sum_{w \in D} {}^2D^4_{i,w} \tau^{10}_{\delta,i} \tau^0_{\delta,\gamma,w} \tau^4_{\delta,\gamma,w} \quad (4r_D r_T^2 N_o) \quad (12223)$$

Raw expression

$${}^2R^4_{j,\zeta} \leftarrow \sum_{\gamma \in A} \sum_{i \in O} \sum_{k \in O} \sum_{l \in O} \sum_{a \in V} \sum_{b \in V} \sum_{c \in V} \sum_{d \in V} \frac{1}{2} \quad (12224)$$

$${}^1T_{b,k} {}^1T_{c,i} Y^{1,*}_{a,\gamma} Y^{2,*}_{i,\gamma} Z^*_{\gamma,\zeta}$$

$$Y^{3,*}_{b,\zeta} {}^2D^{a,i,b,j} {}^2T_{d,j,a,l} V_{k,d,l,c}$$

Factorized expression

$$\tau^0_{\gamma,\delta,w} = \sum_{a \in V} {}^2D^3_{a,w} Y^1_{a,\gamma} Y^{3,*}_{a,\delta} \quad (3r_D r_T^2 N_v) \quad (12225)$$

$$\tau^1_{\gamma,\delta,w} = \sum_{a \in V} {}^2D^1_{a,w} Y^3_{a,\gamma} Y^{1,*}_{a,\delta} \quad (3r_D r_T^2 N_v) \quad (12226)$$

$$\tau^2_{\gamma,\delta,w} = \sum_{i \in O} {}^2D^2_{i,w} Y^4_{i,\gamma} Y^{2,*}_{i,\delta} \quad (3r_D r_T^2 N_o) \quad (12227)$$

$$\tau^3_{\gamma,\delta,w} = \sum_{\epsilon \in A} Z^*_{\epsilon,\delta} \tau^1_{\gamma,\epsilon,w} \tau^2_{\gamma,\epsilon,w} \quad (3r_D r_T^3) \quad (12228)$$

$$\tau^4_{\gamma,\delta,w} = \sum_{\epsilon \in A} Z_{\gamma,\epsilon} \tau^3_{\epsilon,\delta,w} \quad (2r_D r_T^3) \quad (12229)$$

$$\tau^5_{\alpha,i} = \sum_{a \in V} {}^1T_{a,i} W^2_{a,\alpha} \quad (2r_V N_o N_v) \quad (12230)$$

$$\tau^6_{\alpha} = \sum_{i \in O} W^1_{i,\alpha} \tau^5_{\alpha,i} \quad (2r_V N_o) \quad (12231)$$

$$\tau^7_{\alpha} = \sum_{\beta \in B} \tau^6_{\beta} X_{\beta,\alpha} \quad (2r_V^2) \quad (12232)$$

$$\tau^8_{i,a} = \sum_{\alpha \in B} \tau^7_{\alpha} W^3_{i,\alpha} W^4_{a,\alpha} \quad (3r_V N_o N_v) \quad (12233)$$

$$\tau^9_{i,j} = \sum_{a \in V} {}^1T_{a,i} \tau^8_{j,a} \quad (2N_o^2 N_v) \quad (12234)$$

$$\tau^{10}_{\gamma,i} = \sum_{j \in O} Y^2_{j,\gamma} \tau^9_{i,j} \quad (2r_T N_o^2) \quad (12235)$$

$${}^2R^4_{i,\gamma} \leftarrow - \sum_{\delta \in A} \sum_{w \in D} {}^2D^4_{i,w} \tau^{10}_{\delta,i} \tau^0_{\delta,\gamma,w} \tau^4_{\delta,\gamma,w} \quad (4r_D r_T^2 N_o) \quad (12236)$$

Raw expression

$${}^2R^4_{j,\zeta} \leftarrow \sum_{\gamma \in A} \sum_{i \in O} \sum_{k \in O} \sum_{l \in O} \sum_{a \in V} \sum_{b \in V} \sum_{c \in V} \sum_{d \in V} \frac{1}{2} \quad (12237)$$

$${}^1T_{b,k} {}^1T_{c,j} Y^{1,*}_{a,\gamma} Y^{2,*}_{i,\gamma} Z^*_{\gamma,\zeta}$$

$$Y^{3,*}_{b,\zeta} {}^2D^{a,i,b,j} {}^2T_{a,i,d,l} V_{k,d,l,c}$$

Factorized expression

$$\tau^0_{\gamma,w,i} = \sum_{a \in V} {}^2D^3_{a,w} {}^1T_{a,i} Y^{3,*}_{a,\gamma} \quad (3r_D r_T N_o N_v) \quad (12238)$$

$$\tau^1_{\gamma,w,i} = \sum_{a \in V} {}^2D^1_{a,w} {}^1T_{a,i} Y^{1,*}_{a,\gamma} \quad (3r_D r_T N_o N_v) \quad (12239)$$

$$\tau^2_{\gamma,\alpha} = \sum_{a \in V} W^2_{a,\alpha} Y^1_{a,\gamma} \quad (2r_T r_V N_v) \quad (12240)$$

$$\tau^3_{\gamma,\alpha,i} = \sum_{\beta \in B} W^1_{i,\beta} X_{\beta,\alpha} \tau^2_{\gamma,\beta} \quad (3r_T r_V^2 N_o) \quad (12241)$$

$$\tau^4_{\gamma,\alpha} = \sum_{a \in V} W^4_{a,\alpha} Y^3_{a,\gamma} \quad (2r_T r_V N_v) \quad (12242)$$

$$\tau^5_{\gamma,\alpha,i} = \sum_{\delta \in A} Z_{\gamma,\delta} Y^4_{i,\delta} \tau^4_{\delta,\alpha} \quad (3r_T^2 r_V N_o) \quad (12243)$$

$$\tau^6_{\gamma,i,j,k} = \sum_{\alpha \in B} W^3_{j,\alpha} \tau^3_{\gamma,\alpha,i} \tau^5_{\gamma,\alpha,k} \quad (3r_T r_V N_o^3) \quad (12244)$$

$$\tau^7_{i,j,k,l} = \sum_{\gamma \in A} Y^2_{k,\gamma} \tau^6_{\gamma,i,j,l} \quad (2r_T N_o^4) \quad (12245)$$

$$\tau^8_{\gamma,w,i,j} = \sum_{k \in O} \sum_{l \in O} {}^2D^2_{k,w} Y^{2,*}_{k,\gamma} \tau^1_{\gamma,w,l} \tau^7_{l,i,k,j} \quad (4r_D r_T N_o^4) \quad (12246)$$

$$\tau^9_{\gamma,w,i,j} = \sum_{\delta \in A} Z^*_{\delta,\gamma} \tau^8_{\delta,w,i,j} \quad (2r_D r_T^2 N_o^2) \quad (12247)$$

$$\tau^{10}_{\gamma,w,i} = \sum_{j \in O} \tau^0_{\gamma,w,j} \tau^9_{\gamma,w,j,i} \quad (2r_D r_T N_o^2) \quad (12248)$$

$${}^2R^4_{i,\gamma} \leftarrow \sum_{w \in D} \frac{1}{2} {}^2D^4_{i,w} \tau^{10}_{\gamma,w,i} \quad (2r_D r_T N_o) \quad (12249)$$

Raw expression

$${}^2R^4_{j,\zeta} \leftarrow \sum_{\gamma \in A} \sum_{i \in O} \sum_{k \in O} \sum_{l \in O} \sum_{a \in V} \sum_{b \in V} \sum_{c \in V} \sum_{d \in V} \frac{1}{2} \quad (12250)$$

$${}^1T_{b,k} {}^1T_{c,j} Y^{1,*}_{a,\gamma} Y^{2,*}_{i,\gamma} Z^*_{\gamma,\zeta}$$

$$Y^{3,*}_{b,\zeta} {}^2D^{a,i,b,j} {}^2T_{a,l,d,i} V_{k,c,l,d}$$

Factorized expression

$$\tau^0_{\gamma,w,i} = \sum_{a \in V} {}^2D^3_{a,w} {}^1T_{a,i} Y^{3,*}_{a,\gamma} \quad (3r_D r_T N_o N_v) \quad (12251)$$

$$\tau^1_{\gamma,w,i} = \sum_{a \in V} {}^2D^1_{a,w} {}^1T_{a,i} Y^{1,*}_{a,\gamma} \quad (3r_D r_T N_o N_v) \quad (12252)$$

$$\tau^2_{\gamma,\alpha} = \sum_{a \in V} W^4_{a,\alpha} Y^1_{a,\gamma} \quad (2r_T r_V N_v) \quad (12253)$$

$$\tau^3_{\gamma,\alpha,i} = \sum_{\beta \in B} X_{\alpha,\beta} W^3_{i,\beta} \tau^2_{\gamma,\beta} \quad (3r_T r_V^2 N_o) \quad (12254)$$

$$\tau^4_{\gamma,\alpha} = \sum_{a \in V} W^2_{a,\alpha} Y^3_{a,\gamma} \quad (2r_T r_V N_v) \quad (12255)$$

$$\tau^5_{\gamma,\alpha,i} = \sum_{\delta \in A} Z_{\gamma,\delta} Y^4_{i,\delta} \tau^4_{\delta,\alpha} \quad (3r_T^2 r_V N_o) \quad (12256)$$

$$\tau^6_{\gamma,i,j,k} = \sum_{\alpha \in B} W^1_{i,\alpha} \tau^3_{\gamma,\alpha,j} \tau^5_{\gamma,\alpha,k} \quad (3r_T r_V N_o^3) \quad (12257)$$

$$\tau^7_{i,j,k,l} = \sum_{\gamma \in A} Y^2_{k,\gamma} \tau^6_{\gamma,i,j,l} \quad (2r_T N_o^4) \quad (12258)$$

$$\tau^8_{\gamma,w,i,j} = \sum_{k \in O} \sum_{l \in O} {}^2D^2_{k,w} Y^{2,*}_{k,\gamma} \tau^1_{\gamma,w,l} \tau^7_{l,i,j,k} \quad (4r_D r_T N_o^4) \quad (12259)$$

$$\tau^9_{\gamma,w,i,j} = \sum_{\delta \in A} Z^*_{\delta,\gamma} \tau^8_{\delta,w,i,j} \quad (2r_D r_T^2 N_o^2) \quad (12260)$$

$$\tau^{10}_{\gamma,w,i} = \sum_{j \in O} \tau^0_{\gamma,w,j} \tau^9_{\gamma,w,j,i} \quad (2r_D r_T N_o^2) \quad (12261)$$

$${}^2R^4_{i,\gamma} \leftarrow \sum_{w \in D} \frac{1}{2} {}^2D^4_{i,w} \tau^{10}_{\gamma,w,i} \quad (2r_D r_T N_o) \quad (12262)$$

Raw expression

$${}^2R^4_{j,\zeta} \leftarrow \sum_{\gamma \in A} \sum_{i \in O} \sum_{k \in O} \sum_{l \in O} \sum_{a \in V} \sum_{b \in V} \sum_{c \in V} \sum_{d \in V} \frac{1}{2} \quad (12263)$$

$${}^1T_{b,k} {}^1T_{c,j} Y^{1,*}_{a,\gamma} Y^{2,*}_{i,\gamma} Z^*_{\gamma,\zeta}$$

$$Y^{3,*}_{b,\zeta} {}^2D^{a,i,b,j} {}^2T_{d,i,a,l} V_{k,c,l,d}$$

Factorized expression

$$\tau^0_{\gamma,\delta,w} = \sum_{a \in V} {}^2D^3_{a,w} Y^1_{a,\gamma} Y^{3,*}_{a,\delta} \quad (3r_D r_T^2 N_v) \quad (12264)$$

$$\tau^1_{\gamma,\alpha} = \sum_{i \in O} W^3_{i,\alpha} Y^2_{i,\gamma} \quad (2r_T r_V N_o) \quad (12265)$$

$$\tau^2_{\gamma,\alpha} = \sum_{a \in V} W^4_{a,\alpha} Y^3_{a,\gamma} \quad (2r_T r_V N_v) \quad (12266)$$

$$\tau^3_{\gamma,\alpha,i} = \sum_{\delta \in A} Z_{\gamma,\delta} Y^4_{i,\delta} \tau^2_{\delta,\alpha} \quad (3r_T^2 r_V N_o) \quad (12267)$$

$$\tau^4_{\alpha,i} = \sum_{a \in V} {}^1T_{a,i} W^2_{a,\alpha} \quad (2r_V N_o N_v) \quad (12268)$$

$$\tau^5_{\gamma,\alpha,w} = \sum_{i \in O} {}^2D^2_{i,w} Y^{2,*}_{i,\gamma} \tau^4_{\alpha,i} \quad (3r_D r_T r_V N_o) \quad (12269)$$

$$\tau^6_{\gamma,w,i} = \sum_{a \in V} {}^2D^1_{a,w} {}^1T_{a,i} Y^{1,*}_{a,\gamma} \quad (3r_D r_T N_o N_v) \quad (12270)$$

$$\tau^7_{\gamma,\alpha,w} = \sum_{i \in O} W^1_{i,\alpha} \tau^6_{\gamma,w,i} \quad (2r_D r_T r_V N_o) \quad (12271)$$

$$\tau^8_{\gamma,\alpha,w} = \sum_{\beta \in B} X_{\beta,\alpha} \tau^5_{\gamma,\beta,w} \tau^7_{\gamma,\beta,w} \quad (3r_D r_T r_V^2) \quad (12272)$$

$$\tau_{\gamma,\alpha,w}^9 = \sum_{\delta \in A} Z_{\delta,\gamma}^* \tau_{\delta,\alpha,w}^8 \quad (2r_D r_T^2 r_V) \quad (12273)$$

$$\tau_{\gamma,\alpha,w}^7 = \sum_{i \in O} W_{i,\alpha}^1 \tau_{\gamma,w,i}^6 \quad (2r_D r_T r_V N_o) \quad (12285)$$

$$\tau_{\gamma,\delta,w,i}^{10} = \sum_{\alpha \in B} \tau_{\gamma,\alpha}^1 \tau_{\gamma,\alpha,i}^3 \tau_{\delta,\alpha,w}^9 \quad (3r_D r_T^2 r_V N_o) \quad (12274)$$

$$\tau_{\gamma,\alpha,w}^8 = \sum_{\beta \in B} X_{\beta,\alpha} \tau_{\gamma,\beta,w}^5 \tau_{\gamma,\beta,w}^7 \quad (3r_D r_T r_V^2) \quad (12286)$$

$$\tau_{\gamma,w,i}^{11} = \sum_{\delta \in A} \tau_{\delta,\gamma,w}^0 \tau_{\delta,\gamma,w,i}^{10} \quad (2r_D r_T^2 N_o) \quad (12275)$$

$$\tau_{\gamma,\alpha,w}^9 = \sum_{\delta \in A} Z_{\delta,\gamma}^* \tau_{\delta,\alpha,w}^8 \quad (2r_D r_T^2 r_V) \quad (12287)$$

$${}^2R_{i,\gamma}^4 \leftarrow \sum_{w \in D} \frac{1}{2} {}^2D_{i,w}^4 \tau_{\gamma,w,i}^{11} \quad (2r_D r_T N_o) \quad (12276)$$

$$\tau_{\gamma,\delta,w,i}^{10} = \sum_{\alpha \in B} \tau_{\gamma,\alpha}^3 \tau_{\gamma,\alpha,i}^2 \tau_{\delta,\alpha,w}^9 \quad (3r_D r_T^2 r_V N_o) \quad (12288)$$

Raw expression

$${}^2R_{j,\zeta}^4 \leftarrow \sum_{\gamma \in A} \sum_{i \in O} \sum_{k \in O} \sum_{l \in O} \sum_{a \in V} \sum_{b \in V} \sum_{c \in V} \sum_{d \in V} \frac{1}{2} \quad (12277)$$

$$\begin{aligned} & {}^1T_{b,k} \quad {}^1T_{c,j} \quad Y_{a,\gamma}^{1,*} \quad Y_{i,\gamma}^{2,*} \quad Z_{\gamma,\zeta}^* \\ & Y_{b,\zeta}^{3,*} \quad {}^2D_{a,i,b,j} \quad {}^2T_{d,l,a,i} \quad V_{k,d,l,c} \end{aligned}$$

$$\tau_{\gamma,w,i}^{11} = \sum_{\delta \in A} \tau_{\delta,\gamma,w}^0 \tau_{\delta,\gamma,w,i}^{10} \quad (2r_D r_T^2 N_o) \quad (12289)$$

$${}^2R_{i,\gamma}^4 \leftarrow \sum_{w \in D} \frac{1}{2} {}^2D_{i,w}^4 \tau_{\gamma,w,i}^{11} \quad (2r_D r_T N_o) \quad (12290)$$

Factorized expression

$$\tau_{\gamma,\delta,w}^0 = \sum_{a \in V} {}^2D_{a,w}^3 Y_{a,\gamma}^3 Y_{a,\delta}^{3,*} \quad (3r_D r_T^2 N_v) \quad (12278)$$

Raw expression

$${}^2R_{j,\zeta}^4 \leftarrow \sum_{\gamma \in A} \sum_{i \in O} \sum_{k \in O} \sum_{l \in O} \sum_{a \in V} \sum_{b \in V} \sum_{c \in V} \sum_{d \in V} \frac{1}{2} \quad (12291)$$

$$\begin{aligned} & {}^1T_{b,k} \quad {}^1T_{c,l} \quad Y_{a,\gamma}^{1,*} \quad Y_{i,\gamma}^{2,*} \quad Z_{\gamma,\zeta}^* \\ & Y_{b,\zeta}^{3,*} \quad {}^2D_{a,i,b,j} \quad {}^2T_{a,i,d,j} \quad V_{k,c,l,d} \end{aligned}$$

Factorized expression

$$\tau_{\gamma,\alpha}^1 = \sum_{a \in V} W_{a,\alpha}^4 Y_{a,\gamma}^1 \quad (2r_T r_V N_v) \quad (12279)$$

$$\tau_{\gamma,\delta,w}^0 = \sum_{a \in V} {}^2D_{a,w}^3 Y_{a,\gamma}^1 Y_{a,\delta}^{3,*} \quad (3r_D r_T^2 N_v) \quad (12292)$$

$$\tau_{\gamma,\alpha,i}^2 = \sum_{\delta \in A} Y_{i,\delta}^2 Z_{\delta,\gamma} \tau_{\delta,\alpha}^1 \quad (3r_T^2 r_V N_o) \quad (12280)$$

$$\tau_{\gamma,\alpha}^3 = \sum_{i \in O} W_{i,\alpha}^3 Y_{i,\gamma}^4 \quad (2r_T r_V N_o) \quad (12281)$$

$$\tau_{\gamma,w,i}^1 = \sum_{a \in V} {}^2D_{a,w}^1 {}^1T_{a,i} Y_{a,\gamma}^{1,*} \quad (3r_D r_T N_o N_v) \quad (12293)$$

$$\tau_{\alpha,i}^4 = \sum_{a \in V} {}^1T_{a,i} W_{a,\alpha}^2 \quad (2r_V N_o N_v) \quad (12282)$$

$$\tau_{\gamma,\alpha}^2 = \sum_{a \in V} W_{a,\alpha}^2 Y_{a,\gamma}^3 \quad (2r_T r_V N_v) \quad (12294)$$

$$\tau_{\gamma,\alpha,w}^5 = \sum_{i \in O} {}^2D_{i,w}^2 Y_{i,\gamma}^{2,*} \tau_{\alpha,i}^4 \quad (3r_D r_T r_V N_o) \quad (12283)$$

$$\tau_{\alpha,i}^3 = \sum_{a \in V} {}^1T_{a,i} W_{a,\alpha}^4 \quad (2r_V N_o N_v) \quad (12295)$$

$$\tau_{\gamma,w,i}^6 = \sum_{a \in V} {}^2D_{a,w}^1 {}^1T_{a,i} Y_{a,\gamma}^{1,*} \quad (3r_D r_T N_o N_v) \quad (12284)$$

$$\tau_{\alpha,i,j}^4 = \sum_{\beta \in B} X_{\alpha,\beta} W_{j,\beta}^3 \tau_{\beta,i}^3 \quad (3r_V^2 N_o^2) \quad (12296)$$

$$\tau^5_{\gamma,\alpha,i} = \sum_{j \in O} Y^4_{j,\gamma} \tau^4_{\alpha,i,j} \quad (2r_T r_V N_o^2) \quad (12297)$$

$$\tau^5_{\gamma,\alpha,i} = \sum_{j \in O} Y^2_{j,\gamma} \tau^4_{\alpha,i,j} \quad (2r_T r_V N_o^2) \quad (12309)$$

$$\tau^6_{\gamma,i,j} = \sum_{\alpha \in B} W^1_{j,\alpha} \tau^2_{\gamma,\alpha} \tau^5_{\gamma,\alpha,i} \quad (3r_T r_V N_o^2) \quad (12298)$$

$$\tau^6_{\gamma,i,j} = \sum_{\alpha \in B} W^1_{j,\alpha} \tau^2_{\gamma,\alpha} \tau^5_{\gamma,\alpha,i} \quad (3r_T r_V N_o^2) \quad (12310)$$

$$\tau^7_{\gamma,i,j} = \sum_{\delta \in A} Z_{\gamma,\delta} \tau^6_{\delta,i,j} \quad (2r_T^2 N_o^2) \quad (12299)$$

$$\tau^7_{\gamma,i,j} = \sum_{\delta \in A} Z_{\delta,\gamma} \tau^6_{\delta,i,j} \quad (2r_T^2 N_o^2) \quad (12311)$$

$$\tau^8_{\gamma,\delta,w} = \sum_{i \in O} \sum_{j \in O} {}^2D^2_{i,w} Y^{2,*}_{i,\delta} \tau^1_{\delta,w,j} \tau^7_{\gamma,i,j} \quad (4r_D r_T^2 N_o^2) \quad (12300)$$

$$\tau^8_{\gamma,\delta,w} = \sum_{i \in O} \sum_{j \in O} {}^2D^2_{i,w} Y^{2,*}_{i,\delta} \tau^1_{\delta,w,j} \tau^7_{\gamma,i,j} \quad (4r_D r_T^2 N_o^2) \quad (12312)$$

$$\tau^9_{\gamma,\delta,w} = \sum_{\epsilon \in A} Z^*_{\epsilon,\delta} \tau^8_{\gamma,\epsilon,w} \quad (2r_D r_T^3) \quad (12301)$$

$$\tau^9_{\gamma,\delta,w} = \sum_{\epsilon \in A} Z^*_{\epsilon,\delta} \tau^8_{\gamma,\epsilon,w} \quad (2r_D r_T^3) \quad (12313)$$

$${}^2R^4_{i,\gamma} \leftarrow \sum_{\delta \in A} \sum_{w \in D} \frac{1}{2} {}^2D^4_{i,w} Y^2_{i,\delta} \tau^0_{\delta,\gamma,w} \tau^9_{\delta,\gamma,w} \quad (4r_D r_T^2 N_o) \quad (12302)$$

$${}^2R^4_{i,\gamma} \leftarrow \sum_{\delta \in A} \sum_{w \in D} \frac{1}{2} {}^2D^4_{i,w} Y^4_{i,\delta} \tau^0_{\delta,\gamma,w} \tau^9_{\delta,\gamma,w} \quad (4r_D r_T^2 N_o) \quad (12314)$$

Raw expression

$${}^2R^4_{j,\zeta} \leftarrow \sum_{\gamma \in A} \sum_{i \in O} \sum_{k \in O} \sum_{l \in O} \sum_{a \in V} \sum_{b \in V} \sum_{c \in V} \sum_{d \in V} \frac{1}{2} \quad (12303)$$

$$\begin{array}{ccccccc} {}^1T_{b,k} & {}^1T_{c,l} & Y^{1,*}_{a,\gamma} & Y^{2,*}_{i,\gamma} & Z^*_{\gamma,\zeta} & & \\ Y^{3,*}_{b,\zeta} & {}^2D^{a,i,b,j} & {}^2T_{d,j,a,i} & V_{k,c,l,d} & & & \end{array}$$

Raw expression

$${}^2R^4_{j,\zeta} \leftarrow \sum_{\gamma \in A} \sum_{i \in O} \sum_{k \in O} \sum_{l \in O} \sum_{a \in V} \sum_{b \in V} \sum_{c \in V} \sum_{d \in V} \frac{1}{2} \quad (12315)$$

$$\begin{array}{ccccccc} {}^1T_{c,i} & {}^1T_{d,j} & Y^{1,*}_{a,\gamma} & Y^{2,*}_{i,\gamma} & Z^*_{\gamma,\zeta} & & \\ Y^{3,*}_{b,\zeta} & {}^2D^{a,i,b,j} & {}^2T_{a,k,b,l} & V_{k,c,l,d} & & & \end{array}$$

Factorized expression

$$\tau^0_{\gamma,\delta,w} = \sum_{a \in V} {}^2D^3_{a,w} Y^3_{a,\gamma} Y^{3,*}_{a,\delta} \quad (3r_D r_T^2 N_v) \quad (12304)$$

$$\tau^0_{\gamma,\delta,w} = \sum_{a \in V} {}^2D^3_{a,w} Y^1_{a,\gamma} Y^{3,*}_{a,\delta} \quad (3r_D r_T^2 N_v) \quad (12316)$$

$$\tau^1_{\gamma,w,i} = \sum_{a \in V} {}^2D^1_{a,w} {}^1T_{a,i} Y^{1,*}_{a,\gamma} \quad (3r_D r_T N_o N_v) \quad (12305)$$

$$\tau^1_{\alpha,i} = \sum_{a \in V} {}^1T_{a,i} W^4_{a,\alpha} \quad (2r_V N_o N_v) \quad (12317)$$

$$\tau^2_{\gamma,\alpha} = \sum_{a \in V} W^2_{a,\alpha} Y^1_{a,\gamma} \quad (2r_T r_V N_v) \quad (12306)$$

$$\tau^2_{\alpha,i,j} = \sum_{\beta \in B} X_{\alpha,\beta} W^3_{j,\beta} \tau^1_{\beta,i} \quad (3r_V^2 N_o^2) \quad (12318)$$

$$\tau^3_{\alpha,i} = \sum_{a \in V} {}^1T_{a,i} W^4_{a,\alpha} \quad (2r_V N_o N_v) \quad (12307)$$

$$\tau^3_{\gamma,\alpha,i} = \sum_{j \in O} Y^2_{j,\gamma} \tau^2_{\alpha,i,j} \quad (2r_T r_V N_o^2) \quad (12319)$$

$$\tau^4_{\alpha,i,j} = \sum_{\beta \in B} X_{\alpha,\beta} W^3_{j,\beta} \tau^3_{\beta,i} \quad (3r_V^2 N_o^2) \quad (12308)$$

$$\tau^4_{\gamma,w,i} = \sum_{a \in V} {}^2D^1_{a,w} {}^1T_{a,i} Y^{1,*}_{a,\gamma} \quad (3r_D r_T N_o N_v) \quad (12320)$$

$$\tau^5_{\gamma,w,i,j} = \sum_{\delta \in A} {}^2D^2_{i,w} Y^{2,*}_{i,\delta} Z^*_{\delta,\gamma} \tau^4_{\delta,w,j} \quad (4r_D r_T^2 N_o^2) \quad (12321)$$

$$\tau^6_{\gamma,\alpha,w,i} = \sum_{j \in O} W^1_{j,\alpha} \tau^5_{\gamma,w,i,j} \quad (2r_D r_T r_V N_o^2) \quad (12322)$$

$$\tau^7_{\gamma,\alpha} = \sum_{a \in V} W^2_{a,\alpha} Y^3_{a,\gamma} \quad (2r_T r_V N_v) \quad (12323)$$

$$\tau^8_{\gamma,\alpha,i} = \sum_{\delta \in A} Z_{\gamma,\delta} Y^4_{i,\delta} \tau^7_{\delta,\alpha} \quad (3r_T^2 r_V N_o) \quad (12324)$$

$$\tau^9_{\gamma,\delta,\alpha,w} = \sum_{i \in O} \tau^8_{\gamma,\alpha,i} \tau^6_{\delta,\alpha,w,i} \quad (2r_D r_T^2 r_V N_o) \quad (12325)$$

$$\tau^{10}_{\gamma,\delta,w,i} = \sum_{\alpha \in B} \tau^3_{\gamma,\alpha,i} \tau^9_{\gamma,\delta,\alpha,w} \quad (2r_D r_T^2 r_V N_o) \quad (12326)$$

$$\tau^{11}_{\gamma,w,i} = \sum_{\delta \in A} \tau^0_{\delta,\gamma,w} \tau^{10}_{\delta,\gamma,w,i} \quad (2r_D r_T^2 N_o) \quad (12327)$$

$${}^2R^4_{i,\gamma} \leftarrow \sum_{w \in D} \frac{1}{2} {}^2D^4_{i,w} \tau^{11}_{\gamma,w,i} \quad (2r_D r_T N_o) \quad (12328)$$

Raw expression

$${}^2R^4_{j,\zeta} \leftarrow \sum_{\gamma \in A} \sum_{i \in O} \sum_{k \in O} \sum_{l \in O} \sum_{a \in V} \sum_{b \in V} \sum_{c \in V} \sum_{d \in V} \frac{1}{2} \quad (12329)$$

$$\begin{aligned} & {}^1T_{c,i} \quad {}^1T_{d,j} \quad Y^{1,*}_{a,\gamma} \quad Y^{2,*}_{i,\gamma} \quad Z^*_{\gamma,\zeta} \\ & Y^{3,*}_{b,\zeta} \quad {}^2D^{a,i,b,j} \quad {}^2T_{b,k,a,l} \quad V_{k,d,l,c} \end{aligned}$$

Factorized expression

$$\tau^0_{\gamma,\delta,w} = \sum_{a \in V} {}^2D^3_{a,w} Y^3_{a,\gamma} Y^{3,*}_{a,\delta} \quad (3r_D r_T^2 N_v) \quad (12330)$$

$$\tau^1_{\alpha,i} = \sum_{a \in V} {}^1T_{a,i} W^4_{a,\alpha} \quad (2r_V N_o N_v) \quad (12331)$$

$$\tau^2_{\alpha,i,j} = \sum_{\beta \in B} X_{\alpha,\beta} W^3_{j,\beta} \tau^1_{\beta,i} \quad (3r_V^2 N_o^2) \quad (12332)$$

$$\tau^3_{\gamma,\alpha,i} = \sum_{j \in O} Y^4_{j,\gamma} \tau^2_{\alpha,i,j} \quad (2r_T r_V N_o^2) \quad (12333)$$

$$\tau^4_{\gamma,w,i} = \sum_{a \in V} {}^2D^1_{a,w} {}^1T_{a,i} Y^{1,*}_{a,\gamma} \quad (3r_D r_T N_o N_v) \quad (12334)$$

$$\tau^5_{\gamma,w,i,j} = \sum_{\delta \in A} {}^2D^2_{i,w} Y^{2,*}_{i,\delta} Z^*_{\delta,\gamma} \tau^4_{\delta,w,j} \quad (4r_D r_T^2 N_o^2) \quad (12335)$$

$$\tau^6_{\gamma,\alpha,w,i} = \sum_{j \in O} W^1_{j,\alpha} \tau^5_{\gamma,w,i,j} \quad (2r_D r_T r_V N_o^2) \quad (12336)$$

$$\tau^7_{\gamma,\alpha} = \sum_{a \in V} W^2_{a,\alpha} Y^1_{a,\gamma} \quad (2r_T r_V N_v) \quad (12337)$$

$$\tau^8_{\gamma,\alpha,i} = \sum_{\delta \in A} Y^2_{i,\delta} Z_{\delta,\gamma} \tau^7_{\delta,\alpha} \quad (3r_T^2 r_V N_o) \quad (12338)$$

$$\tau^9_{\gamma,\delta,\alpha,w} = \sum_{i \in O} \tau^8_{\gamma,\alpha,i} \tau^6_{\delta,\alpha,w,i} \quad (2r_D r_T^2 r_V N_o) \quad (12339)$$

$$\tau^{10}_{\gamma,\delta,w,i} = \sum_{\alpha \in B} \tau^3_{\gamma,\alpha,i} \tau^9_{\gamma,\delta,\alpha,w} \quad (2r_D r_T^2 r_V N_o) \quad (12340)$$

$$\tau^{11}_{\gamma,w,i} = \sum_{\delta \in A} \tau^0_{\delta,\gamma,w} \tau^{10}_{\delta,\gamma,w,i} \quad (2r_D r_T^2 N_o) \quad (12341)$$

$${}^2R^4_{i,\gamma} \leftarrow \sum_{w \in D} \frac{1}{2} {}^2D^4_{i,w} \tau^{11}_{\gamma,w,i} \quad (2r_D r_T N_o) \quad (12342)$$

Raw expression

$${}^2R^4_{j,\zeta} \leftarrow \sum_{\gamma \in A} \sum_{i \in O} \sum_{k \in O} \sum_{l \in O} \sum_{a \in V} \sum_{b \in V} \sum_{c \in V} \sum_{d \in V} \frac{1}{2} \quad (12343)$$

$$\begin{aligned} & {}^1T_{c,i} \quad {}^1T_{d,k} \quad Y^{1,*}_{a,\gamma} \quad Y^{2,*}_{i,\gamma} \quad Z^*_{\gamma,\zeta} \\ & Y^{3,*}_{b,\zeta} \quad {}^2D^{a,i,b,j} \quad {}^2T_{a,l,b,j} \quad V_{k,c,l,d} \end{aligned}$$

Factorized expression

$$\tau^0_{\gamma,\delta,w} = \sum_{a \in V} {}^2D^3_{a,w} Y^1_{a,\gamma} Y^{3,*}_{a,\delta} \quad (3r_D r_T^2 N_v) \quad (12344)$$

$$\tau^1_{\gamma,\delta,w} = \sum_{i \in O} {}^2D^2_{i,w} Y^4_{i,\gamma} Y^{2,*}_{i,\delta} \quad (3r_D r_T^2 N_o) \quad (12345)$$

$$\tau^1_{\gamma,\delta,w} = \sum_{i \in O} {}^2D^2_{i,w} Y^2_{i,\gamma} Y^{2,*}_{i,\delta} \quad (3r_D r_T^2 N_o) \quad (12358)$$

$$\tau^2_{\gamma,w,i} = \sum_{a \in V} {}^2D^1_{a,w} {}^1T_{a,i} Y^{1,*}_{a,\gamma} \quad (3r_D r_T N_o N_v) \quad (12346)$$

$$\tau^2_{\gamma,w,i} = \sum_{a \in V} {}^2D^1_{a,w} {}^1T_{a,i} Y^{1,*}_{a,\gamma} \quad (3r_D r_T N_o N_v) \quad (12359)$$

$$\tau^3_{\alpha,i} = \sum_{a \in V} {}^1T_{a,i} W^2_{a,\alpha} \quad (2r_V N_o N_v) \quad (12347)$$

$$\tau^3_{\alpha,i} = \sum_{a \in V} {}^1T_{a,i} W^2_{a,\alpha} \quad (2r_V N_o N_v) \quad (12360)$$

$$\tau^4_{\alpha,\beta} = \sum_{i \in O} W^3_{i,\beta} \tau^3_{\alpha,i} \quad (2r_V^2 N_o) \quad (12348)$$

$$\tau^4_{\alpha,\beta} = \sum_{i \in O} W^3_{i,\beta} \tau^3_{\alpha,i} \quad (2r_V^2 N_o) \quad (12361)$$

$$\tau^5_{\alpha,i} = \sum_{\beta \in B} W^1_{i,\beta} X_{\beta,\alpha} \tau^4_{\beta,\alpha} \quad (3r_V^2 N_o) \quad (12349)$$

$$\tau^5_{\alpha,i} = \sum_{\beta \in B} W^1_{i,\beta} X_{\beta,\alpha} \tau^4_{\beta,\alpha} \quad (3r_V^2 N_o) \quad (12362)$$

$$\tau^6_{i,a} = \sum_{\alpha \in B} W^4_{a,\alpha} \tau^5_{\alpha,i} \quad (2r_V N_o N_v) \quad (12350)$$

$$\tau^6_{i,a} = \sum_{\alpha \in B} W^4_{a,\alpha} \tau^5_{\alpha,i} \quad (2r_V N_o N_v) \quad (12363)$$

$$\tau^7_{\gamma,i} = \sum_{a \in V} Y^3_{a,\gamma} \tau^6_{i,a} \quad (2r_T N_o N_v) \quad (12351)$$

$$\tau^7_{\gamma,i} = \sum_{a \in V} Y^1_{a,\gamma} \tau^6_{i,a} \quad (2r_T N_o N_v) \quad (12364)$$

$$\tau^8_{\gamma,\delta,w} = \sum_{i \in O} \tau^7_{\gamma,i} \tau^2_{\delta,w,i} \quad (2r_D r_T^2 N_o) \quad (12352)$$

$$\tau^8_{\gamma,\delta,w} = \sum_{i \in O} \tau^7_{\gamma,i} \tau^2_{\delta,w,i} \quad (2r_D r_T^2 N_o) \quad (12365)$$

$$\tau^9_{\gamma,\delta,w} = \sum_{\epsilon \in A} Z^*_{\epsilon,\delta} \tau^1_{\gamma,\epsilon,w} \tau^8_{\gamma,\epsilon,w} \quad (3r_D r_T^3) \quad (12353)$$

$$\tau^9_{\gamma,\delta,w} = \sum_{\epsilon \in A} Z^*_{\epsilon,\delta} \tau^1_{\gamma,\epsilon,w} \tau^8_{\gamma,\epsilon,w} \quad (3r_D r_T^3) \quad (12366)$$

$$\tau^{10}_{\gamma,\delta,w} = \sum_{\epsilon \in A} Z_{\gamma,\epsilon} \tau^9_{\epsilon,\delta,w} \quad (2r_D r_T^3) \quad (12354)$$

$$\tau^{10}_{\gamma,\delta,w} = \sum_{\epsilon \in A} Z_{\epsilon,\gamma} \tau^9_{\epsilon,\delta,w} \quad (2r_D r_T^3) \quad (12367)$$

$${}^2R^4_{i,\gamma} \leftarrow \sum_{\delta \in A} \sum_{w \in D} \frac{1}{2} {}^2D^4_{i,w} Y^2_{i,\delta} \tau^0_{\delta,\gamma,w} \tau^{10}_{\delta,\gamma,w} \quad (4r_D r_T^2 N_o) \quad (12355)$$

$${}^2R^4_{i,\gamma} \leftarrow \sum_{\delta \in A} \sum_{w \in D} \frac{1}{2} {}^2D^4_{i,w} Y^4_{i,\delta} \tau^0_{\delta,\gamma,w} \tau^{10}_{\delta,\gamma,w} \quad (4r_D r_T^2 N_o) \quad (12368)$$

Raw expression

$${}^2R^4_{j,\zeta} \leftarrow \sum_{\gamma \in A} \sum_{i \in O} \sum_{k \in O} \sum_{l \in O} \sum_{a \in V} \sum_{b \in V} \sum_{c \in V} \sum_{d \in V} \frac{1}{2} \quad (12356)$$

$${}^1T_{c,i} {}^1T_{d,k} Y^{1,*}_{a,\gamma} Y^{2,*}_{i,\gamma} Z^*_{\gamma,\zeta} Y^{3,*}_{b,\zeta} {}^2D^{a,i,b,j} {}^2T_{b,j,a,l} V_{k,c,l,d}$$

Raw expression

$${}^2R^4_{j,\zeta} \leftarrow \sum_{\gamma \in A} \sum_{i \in O} \sum_{k \in O} \sum_{l \in O} \sum_{a \in V} \sum_{b \in V} \sum_{c \in V} \sum_{d \in V} \frac{1}{2} \quad (12369)$$

$${}^1T_{c,k} {}^1T_{d,j} Y^{1,*}_{a,\gamma} Y^{2,*}_{i,\gamma} Z^*_{\gamma,\zeta} Y^{3,*}_{b,\zeta} {}^2D^{a,i,b,j} {}^2T_{a,i,b,l} V_{k,d,l,c}$$

Factorized expression

$$\tau^0_{\gamma,\delta,w} = \sum_{a \in V} {}^2D^3_{a,w} Y^3_{a,\gamma} Y^{3,*}_{a,\delta} \quad (3r_D r_T^2 N_v) \quad (12357)$$

Factorized expression

$$\tau^0_{\gamma,w,i} = \sum_{a \in V} {}^2D^3_{a,w} {}^1T_{a,i} Y^{3,*}_{a,\gamma} \quad (3r_D r_T N_o N_v) \quad (12370)$$



$$\tau^1_{\gamma,\alpha} = \sum_{a \in V} W^2_{a,\alpha} Y^3_{a,\gamma} \quad (2r_T r_V N_v) \quad (12371)$$

$$\tau^2_{\gamma,\alpha,i} = \sum_{\delta \in A} Z_{\gamma,\delta} Y^4_{i,\delta} \tau^1_{\delta,\alpha} \quad (3r_T^2 r_V N_o) \quad (12372)$$

$$\tau^3_{\gamma,\delta,w} = \sum_{a \in V} {}^2D^1_{a,w} Y^1_{a,\gamma} Y^{1,*}_{a,\delta} \quad (3r_D r_T^2 N_v) \quad (12373)$$

$$\tau^4_{\alpha,i} = \sum_{a \in V} {}^1T_{a,i} W^4_{a,\alpha} \quad (2r_V N_o N_v) \quad (12374)$$

$$\tau^5_{\alpha,i,j} = \sum_{\beta \in B} X_{\alpha,\beta} W^3_{j,\beta} \tau^4_{\beta,i} \quad (3r_V^2 N_o^2) \quad (12375)$$

$$\tau^6_{\gamma,\alpha,i} = \sum_{j \in O} Y^2_{j,\gamma} \tau^5_{\alpha,i,j} \quad (2r_T r_V N_o^2) \quad (12376)$$

$$\tau^7_{\gamma,\delta,\alpha,w} = \sum_{i \in O} {}^2D^2_{i,w} Y^{2,*}_{i,\delta} \tau^3_{\gamma,\delta,w} \tau^6_{\gamma,\alpha,i} \quad (4r_D r_T^2 r_V N_o) \quad (12377)$$

$$\tau^8_{\gamma,\alpha,w,i} = \sum_{\delta \in A} \tau^2_{\delta,\alpha,i} \tau^7_{\delta,\gamma,\alpha,w} \quad (2r_D r_T^2 r_V N_o) \quad (12378)$$

$$\tau^9_{\gamma,w,i,j} = \sum_{\alpha \in B} W^1_{i,\alpha} \tau^8_{\gamma,\alpha,w,j} \quad (2r_D r_T r_V N_o^2) \quad (12379)$$

$$\tau^{10}_{\gamma,w,i,j} = \sum_{\delta \in A} Z^*_{\delta,\gamma} \tau^9_{\delta,w,i,j} \quad (2r_D r_T^2 N_o^2) \quad (12380)$$

$$\tau^{11}_{\gamma,w,i} = \sum_{j \in O} \tau^0_{\gamma,w,j} \tau^{10}_{\gamma,w,j,i} \quad (2r_D r_T N_o^2) \quad (12381)$$

$${}^2R^4_{i,\gamma} \leftarrow \sum_{w \in D} \frac{1}{2} {}^2D^4_{i,w} \tau^{11}_{\gamma,w,i} \quad (2r_D r_T N_o) \quad (12382)$$

Raw expression

$${}^2R^4_{j,\zeta} \leftarrow \sum_{\gamma \in A} \sum_{i \in O} \sum_{k \in O} \sum_{l \in O} \sum_{a \in V} \sum_{b \in V} \sum_{c \in V} \sum_{d \in V} \frac{1}{2} \quad (12383)$$

$${}^1T_{c,k} \quad {}^1T_{d,j} \quad Y^{1,*}_{a,\gamma} \quad Y^{2,*}_{i,\gamma} \quad Z^*_{\gamma,\zeta} \quad Y^{3,*}_{b,\zeta} \quad {}^2D^{a,i,b,j}_{a,i} \quad {}^2T_{b,l,a,i} \quad V_{k,d,l,c}$$

Factorized expression

$$\tau^0_{\gamma,w,i} = \sum_{a \in V} {}^2D^3_{a,w} {}^1T_{a,i} Y^{3,*}_{a,\gamma} \quad (3r_D r_T N_o N_v) \quad (12384)$$

$$\tau^1_{\gamma,\alpha} = \sum_{a \in V} W^2_{a,\alpha} Y^1_{a,\gamma} \quad (2r_T r_V N_v) \quad (12385)$$

$$\tau^2_{\gamma,\alpha,i} = \sum_{\delta \in A} Y^2_{i,\delta} Z_{\delta,\gamma} \tau^1_{\delta,\alpha} \quad (3r_T^2 r_V N_o) \quad (12386)$$

$$\tau^3_{\gamma,\delta,w} = \sum_{a \in V} {}^2D^1_{a,w} Y^3_{a,\gamma} Y^{1,*}_{a,\delta} \quad (3r_D r_T^2 N_v) \quad (12387)$$

$$\tau^4_{\alpha,i} = \sum_{a \in V} {}^1T_{a,i} W^4_{a,\alpha} \quad (2r_V N_o N_v) \quad (12388)$$

$$\tau^5_{\alpha,i,j} = \sum_{\beta \in B} X_{\alpha,\beta} W^3_{j,\beta} \tau^4_{\beta,i} \quad (3r_V^2 N_o^2) \quad (12389)$$

$$\tau^6_{\gamma,\alpha,i} = \sum_{j \in O} Y^4_{j,\gamma} \tau^5_{\alpha,i,j} \quad (2r_T r_V N_o^2) \quad (12390)$$

$$\tau^7_{\gamma,\delta,\alpha,w} = \sum_{i \in O} {}^2D^2_{i,w} Y^{2,*}_{i,\delta} \tau^3_{\gamma,\delta,w} \tau^6_{\gamma,\alpha,i} \quad (4r_D r_T^2 r_V N_o) \quad (12391)$$

$$\tau^8_{\gamma,\alpha,w,i} = \sum_{\delta \in A} \tau^2_{\delta,\alpha,i} \tau^7_{\delta,\gamma,\alpha,w} \quad (2r_D r_T^2 r_V N_o) \quad (12392)$$

$$\tau^9_{\gamma,w,i,j} = \sum_{\alpha \in B} W^1_{i,\alpha} \tau^8_{\gamma,\alpha,w,j} \quad (2r_D r_T r_V N_o^2) \quad (12393)$$

$$\tau^{10}_{\gamma,w,i,j} = \sum_{\delta \in A} Z^*_{\delta,\gamma} \tau^9_{\delta,w,i,j} \quad (2r_D r_T^2 N_o^2) \quad (12394)$$

$$\tau^{11}_{\gamma,w,i} = \sum_{j \in O} \tau^0_{\gamma,w,j} \tau^{10}_{\gamma,w,j,i} \quad (2r_D r_T N_o^2) \quad (12395)$$

$${}^2R^4_{i,\gamma} \leftarrow \sum_{w \in D} \frac{1}{2} {}^2D^4_{i,w} \tau^{11}_{\gamma,w,i} \quad (2r_D r_T N_o) \quad (12396)$$

Raw expression

$${}^2R^4_{j,\zeta} \leftarrow - \sum_{\gamma \in A} \sum_{i \in O} \sum_{k \in O} \sum_{l \in O} \sum_{a \in V} \sum_{b \in V} \sum_{c \in V} \sum_{d \in V} {}^1T_{a,k} \\ {}^1T_{c,i} Y^{1,*}_{a,\gamma} Y^{2,*}_{i,\gamma} Z^*_{\gamma,\zeta} \\ Y^{3,*}_{b,\zeta} {}^2D^{a,i,b,j} {}^2T_{b,j,d,l} V_{k,c,l,d} \quad (12397)$$

Factorized expression

$$\tau^0_{\gamma,w,i} = \sum_{a \in V} {}^2D^3_{a,w} {}^1T_{a,i} Y^{3,*}_{a,\gamma} \quad (3r_D r_T N_o N_v) \quad (12398)$$

$$\tau^1_{\gamma,\alpha,w} = \sum_{i \in O} W^1_{i,\alpha} \tau^0_{\gamma,w,i} \quad (2r_D r_T r_V N_o) \quad (12399)$$

$$\tau^2_{\gamma,\delta,w} = \sum_{a \in V} {}^2D^1_{a,w} Y^1_{a,\gamma} Y^{1,*}_{a,\delta} \quad (3r_D r_T^2 N_v) \quad (12400)$$

$$\tau^3_{\gamma,\alpha} = \sum_{i \in O} W^3_{i,\alpha} Y^2_{i,\gamma} \quad (2r_T r_V N_o) \quad (12401)$$

$$\tau^4_{\gamma,\alpha} = \sum_{a \in V} W^4_{a,\alpha} Y^3_{a,\gamma} \quad (2r_T r_V N_v) \quad (12402)$$

$$\tau^5_{\gamma,\alpha,i} = \sum_{\delta \in A} Z_{\gamma,\delta} Y^4_{i,\delta} \tau^4_{\delta,\alpha} \quad (3r_T^2 r_V N_o) \quad (12403)$$

$$\tau^6_{\gamma,\alpha,w} = \sum_{\delta \in A} \sum_{i \in O} {}^2D^2_{i,w} Y^{2,*}_{i,\gamma} \tau^3_{\delta,\alpha} \tau^2_{\delta,\gamma,w} \tau^5_{\delta,\alpha,i} \quad (5r_D r_T^2 r_V N_o) \quad (12404)$$

$$\tau^7_{\gamma,\alpha,w} = \sum_{\beta \in B} X_{\alpha,\beta} \tau^6_{\gamma,\beta,w} \quad (2r_D r_T r_V^2) \quad (12405)$$

$$\tau^8_{\gamma,\alpha,w} = \sum_{\delta \in A} Z^*_{\delta,\gamma} \tau^7_{\delta,\alpha,w} \quad (2r_D r_T^2 r_V) \quad (12406)$$

$$\tau^9_{\alpha,i} = \sum_{a \in V} {}^1T_{a,i} W^2_{a,\alpha} \quad (2r_V N_o N_v) \quad (12407)$$

$$\tau^{10}_{\gamma,w,i} = \sum_{\alpha \in B} \tau^9_{\alpha,i} \tau^1_{\gamma,\alpha,w} \tau^8_{\gamma,\alpha,w} \quad (3r_D r_T r_V N_o) \quad (12408)$$

$${}^2R^4_{i,\gamma} \leftarrow \sum_{w \in D} \frac{1}{2} {}^2D^4_{i,w} \tau^{10}_{\gamma,w,i} \quad (2r_D r_T N_o) \quad (12409)$$

Raw expression

$${}^2R^4_{j,\zeta} \leftarrow - \sum_{\gamma \in A} \sum_{i \in O} \sum_{k \in O} \sum_{l \in O} \sum_{a \in V} \sum_{b \in V} \sum_{c \in V} \sum_{d \in V} {}^1T_{a,k} \\ {}^1T_{c,i} Y^{1,*}_{a,\gamma} Y^{2,*}_{i,\gamma} Z^*_{\gamma,\zeta} \\ Y^{3,*}_{b,\zeta} {}^2D^{a,i,b,j} {}^2T_{d,l,b,j} V_{k,c,l,d} \quad (12410)$$

Factorized expression

$$\tau^0_{\gamma,w,i} = \sum_{a \in V} {}^2D^3_{a,w} {}^1T_{a,i} Y^{3,*}_{a,\gamma} \quad (3r_D r_T N_o N_v) \quad (12411)$$

$$\tau^1_{\gamma,\alpha,w} = \sum_{i \in O} W^1_{i,\alpha} \tau^0_{\gamma,w,i} \quad (2r_D r_T r_V N_o) \quad (12412)$$

$$\tau^2_{\gamma,\delta,w} = \sum_{a \in V} {}^2D^1_{a,w} Y^3_{a,\gamma} Y^{1,*}_{a,\delta} \quad (3r_D r_T^2 N_v) \quad (12413)$$

$$\tau^3_{\gamma,\alpha} = \sum_{a \in V} W^4_{a,\alpha} Y^1_{a,\gamma} \quad (2r_T r_V N_v) \quad (12414)$$

$$\tau^4_{\gamma,\alpha,i} = \sum_{\delta \in A} Y^2_{i,\delta} Z_{\delta,\gamma} \tau^3_{\delta,\alpha} \quad (3r_T^2 r_V N_o) \quad (12415)$$

$$\tau^5_{\gamma,\alpha} = \sum_{i \in O} W^3_{i,\alpha} Y^4_{i,\gamma} \quad (2r_T r_V N_o) \quad (12416)$$

$$\tau^6_{\gamma,\alpha,w} = \sum_{\delta \in A} \sum_{i \in O} {}^2D^2_{i,w} Y^{2,*}_{i,\gamma} \tau^5_{\delta,\alpha} \tau^2_{\delta,\gamma,w} \tau^4_{\delta,\alpha,i} \quad (5r_D r_T^2 r_V N_o) \quad (12417)$$

$$\tau^7_{\gamma,\alpha,w} = \sum_{\beta \in B} X_{\alpha,\beta} \tau^6_{\gamma,\beta,w} \quad (2r_D r_T r_V^2) \quad (12418)$$

$$\tau^8_{\gamma,\alpha,w} = \sum_{\delta \in A} Z^*_{\delta,\gamma} \tau^7_{\delta,\alpha,w} \quad (2r_D r_T^2 r_V) \quad (12419)$$

$$\tau^9_{\alpha,i} = \sum_{a \in V} {}^1T_{a,i} W^2_{a,\alpha} \quad (2r_V N_o N_v) \quad (12420)$$

$$\tau^{10}_{\gamma,w,i} = \sum_{\alpha \in B} \tau^9_{\alpha,i} \tau^1_{\gamma,\alpha,w} \tau^8_{\gamma,\alpha,w} \quad (3r_D r_T r_V N_o) \quad (12421)$$

$${}^2R^4_{i,\gamma} \leftarrow \sum_{w \in D} \frac{1}{2} {}^2D^4_{i,w} \tau^{10}_{\gamma,w,i} \quad (2r_D r_T N_o) \quad (12422)$$

Raw expression

$${}^2R^4_{j,\zeta} \leftarrow - \sum_{\gamma \in A} \sum_{i \in O} \sum_{k \in O} \sum_{l \in O} \sum_{a \in V} \sum_{b \in V} \sum_{c \in V} \sum_{d \in V} {}^1T_{a,k} \\ {}^1T_{c,l} Y^{1,*}_{a,\gamma} Y^{2,*}_{i,\gamma} Z^*_{\gamma,\zeta} \\ Y^{3,*}_{b,\zeta} {}^2D^{a,i,b,j} {}^2T_{b,j,d,i} V_{k,d,l,c} \quad (12423)$$

Factorized expression

$$\tau^0_{\gamma,w,i} = \sum_{a \in V} {}^2D^3_{a,w} {}^1T_{a,i} Y^{3,*}_{a,\gamma} \quad (3r_D r_T N_o N_v) \quad (12424)$$

$$\tau^1_{\gamma,\alpha} = \sum_{a \in V} W^2_{a,\alpha} Y^3_{a,\gamma} \quad (2r_T r_V N_v) \quad (12425)$$

$$\tau^2_{\alpha,i} = \sum_{a \in V} {}^1T_{a,i} W^4_{a,\alpha} \quad (2r_V N_o N_v) \quad (12426)$$

$$\tau^3_{\alpha,i,j} = \sum_{\beta \in B} X_{\alpha,\beta} W^3_{j,\beta} \tau^2_{\beta,i} \quad (3r_V^2 N_o^2) \quad (12427)$$

$$\tau^4_{\gamma,\alpha,i} = \sum_{j \in O} Y^4_{j,\gamma} \tau^3_{\alpha,i,j} \quad (2r_T r_V N_o^2) \quad (12428)$$

$$\tau^5_{\gamma,i,j} = \sum_{\alpha \in B} W^1_{j,\alpha} \tau^1_{\gamma,\alpha} \tau^4_{\gamma,\alpha,i} \quad (3r_T r_V N_o^2) \quad (12429)$$

$$\tau^6_{\gamma,i,j} = \sum_{\delta \in A} Z_{\gamma,\delta} \tau^5_{\delta,i,j} \quad (2r_T^2 N_o^2) \quad (12430)$$

$$\tau^7_{\gamma,\delta,w} = \sum_{a \in V} {}^2D^1_{a,w} Y^1_{a,\gamma} Y^{1,*}_{a,\delta} \quad (3r_D r_T^2 N_v) \quad (12431)$$

$$\tau^8_{\gamma,\delta,w} = \sum_{i \in O} {}^2D^2_{i,w} Y^2_{i,\gamma} Y^{2,*}_{i,\delta} \quad (3r_D r_T^2 N_o) \quad (12432)$$

$$\tau^9_{\gamma,\delta,w} = \sum_{\epsilon \in A} Z^*_{\epsilon,\delta} \tau^7_{\gamma,\epsilon,w} \tau^8_{\gamma,\epsilon,w} \quad (3r_D r_T^3) \quad (12433)$$

$$\tau^{10}_{\gamma,w,i,j} = \sum_{\delta \in A} \tau^6_{\delta,i,j} \tau^9_{\delta,\gamma,w} \quad (2r_D r_T^2 N_o^2) \quad (12434)$$

$$\tau^{11}_{\gamma,w,i} = \sum_{j \in O} \tau^0_{\gamma,w,j} \tau^{10}_{\gamma,w,i,j} \quad (2r_D r_T N_o^2) \quad (12435)$$

$${}^2R^4_{i,\gamma} \leftarrow \sum_{w \in D} \frac{1}{2} {}^2D^4_{i,w} \tau^{11}_{\gamma,w,i} \quad (2r_D r_T N_o) \quad (12436)$$

Raw expression

$${}^2R^4_{j,\zeta} \leftarrow - \sum_{\gamma \in A} \sum_{i \in O} \sum_{k \in O} \sum_{l \in O} \sum_{a \in V} \sum_{b \in V} \sum_{c \in V} \sum_{d \in V} {}^1T_{a,k} \\ {}^1T_{c,l} Y^{1,*}_{a,\gamma} Y^{2,*}_{i,\gamma} Z^*_{\gamma,\zeta} \\ Y^{3,*}_{b,\zeta} {}^2D^{a,i,b,j} {}^2T_{d,i,b,j} V_{k,d,l,c} \quad (12437)$$

Factorized expression

$$\tau^0_{\gamma,w,i} = \sum_{a \in V} {}^2D^3_{a,w} {}^1T_{a,i} Y^{3,*}_{a,\gamma} \quad (3r_D r_T N_o N_v) \quad (12438)$$

$$\tau^1_{\gamma,\alpha} = \sum_{a \in V} W^2_{a,\alpha} Y^1_{a,\gamma} \quad (2r_T r_V N_v) \quad (12439)$$

$$\tau^2_{\alpha,i} = \sum_{a \in V} {}^1T_{a,i} W^4_{a,\alpha} \quad (2r_V N_o N_v) \quad (12440)$$

$$\tau^3_{\alpha,i,j} = \sum_{\beta \in B} X_{\alpha,\beta} W^3_{j,\beta} \tau^2_{\beta,i} \quad (3r_V^2 N_o^2) \quad (12441)$$

$$\tau^4_{\gamma,\alpha,i} = \sum_{j \in O} Y^2_{j,\gamma} \tau^3_{\alpha,i,j} \quad (2r_T r_V N_o^2) \quad (12442)$$

$$\tau^5_{\gamma,i,j} = \sum_{\alpha \in B} W^1_{j,\alpha} \tau^1_{\gamma,\alpha} \tau^4_{\gamma,\alpha,i} \quad (3r_T r_V N_o^2) \quad (12443)$$

$$\tau^6_{\gamma,i,j} = \sum_{\delta \in A} Z_{\delta,\gamma} \tau^5_{\delta,i,j} \quad (2r_T^2 N_o^2) \quad (12444)$$

$$\tau^7_{\gamma,\delta,w} = \sum_{a \in V} {}^2D^1_{a,w} Y^3_{a,\gamma} Y^{1,*}_{a,\delta} \quad (3r_D r_T^2 N_v) \quad (12445)$$

$$\tau^8_{\gamma,\delta,w} = \sum_{i \in O} {}^2D^2_{i,w} Y^4_{i,\gamma} Y^{2,*}_{i,\delta} \quad (3r_D r_T^2 N_o) \quad (12446)$$

$$\tau^9_{\gamma,\delta,w} = \sum_{\epsilon \in A} Z^*_{\epsilon,\delta} \tau^7_{\gamma,\epsilon,w} \tau^8_{\gamma,\epsilon,w} \quad (3r_D r_T^3) \quad (12447)$$

$$\tau_{\gamma,w,i,j}^{10} = \sum_{\delta \in A} \tau_{\delta,i,j}^6 \tau_{\delta,\gamma,w}^9 \quad (2r_D r_T^2 N_o^2) \quad (12448)$$

$$\tau_{\gamma,\delta,w}^9 = \sum_{\epsilon \in A} Z_{\epsilon,\delta}^* \tau_{\gamma,\epsilon,w}^7 \tau_{\gamma,\epsilon,w}^8 \quad (3r_D r_T^3) \quad (12461)$$

$$\tau_{\gamma,w,i}^{11} = \sum_{j \in O} \tau_{\gamma,w,j}^0 \tau_{\gamma,w,i,j}^{10} \quad (2r_D r_T N_o^2) \quad (12449)$$

$$\tau_{\gamma,\delta,w}^{10} = \sum_{\epsilon \in A} Z_{\epsilon,\gamma} \tau_{\epsilon,\delta,w}^9 \quad (2r_D r_T^3) \quad (12462)$$

$${}^2R_{i,\gamma}^4 \leftarrow \sum_{w \in D} \frac{1}{2} {}^2D_{i,w}^4 \tau_{\gamma,w,i}^{11} \quad (2r_D r_T N_o) \quad (12450)$$

$${}^2R_{i,\gamma}^4 \leftarrow \sum_{\delta \in A} \sum_{w \in D} \frac{1}{2} {}^2D_{i,w}^4 Y_{i,\delta}^4 \tau_{\delta,\gamma,w}^{10} \tau_{\delta,\gamma,w}^6 \quad (4r_D r_T^2 N_o) \quad (12463)$$

Raw expression

$$\begin{aligned} {}^2R_{j,\zeta}^4 \leftarrow & - \sum_{\gamma \in A} \sum_{i \in O} \sum_{k \in O} \sum_{l \in O} \sum_{a \in V} \sum_{b \in V} \sum_{c \in V} \sum_{d \in V} {}^1T_{b,k} \\ & {}^1T_{c,j} Y_{a,\gamma}^{1,*} Y_{i,\gamma}^{2,*} Z_{\gamma,\zeta}^* \\ & Y_{b,\zeta}^{3,*} {}^2D_{a,i,b,j} {}^2T_{a,i,d,l} V_{k,c,l,d} \end{aligned} \quad (12451)$$

Raw expression

$$\begin{aligned} {}^2R_{j,\zeta}^4 \leftarrow & - \sum_{\gamma \in A} \sum_{i \in O} \sum_{k \in O} \sum_{l \in O} \sum_{a \in V} \sum_{b \in V} \sum_{c \in V} \sum_{d \in V} {}^1T_{b,k} \\ & {}^1T_{c,j} Y_{a,\gamma}^{1,*} Y_{i,\gamma}^{2,*} Z_{\gamma,\zeta}^* \\ & Y_{b,\zeta}^{3,*} {}^2D_{a,i,b,j} {}^2T_{d,l,a,i} V_{k,c,l,d} \end{aligned} \quad (12464)$$

Factorized expression

$$\tau_{\gamma,w,i}^0 = \sum_{a \in V} {}^2D_{a,w}^3 {}^1T_{a,i} Y_{a,\gamma}^{3,*} \quad (3r_D r_T N_o N_v) \quad (12452)$$

Factorized expression

$$\tau_{\gamma,w,i}^0 = \sum_{a \in V} {}^2D_{a,w}^3 {}^1T_{a,i} Y_{a,\gamma}^{3,*} \quad (3r_D r_T N_o N_v) \quad (12465)$$

$$\tau_{\alpha,i}^1 = \sum_{a \in V} {}^1T_{a,i} W_{a,\alpha}^2 \quad (2r_V N_o N_v) \quad (12453)$$

$$\tau_{\alpha,i}^1 = \sum_{a \in V} {}^1T_{a,i} W_{a,\alpha}^2 \quad (2r_V N_o N_v) \quad (12466)$$

$$\tau_{\alpha,\beta}^2 = \sum_{i \in O} W_{i,\beta}^3 \tau_{\alpha,i}^1 \quad (2r_V^2 N_o) \quad (12454)$$

$$\tau_{\alpha,\beta}^2 = \sum_{i \in O} W_{i,\beta}^3 \tau_{\alpha,i}^1 \quad (2r_V^2 N_o) \quad (12467)$$

$$\tau_{\alpha,i}^3 = \sum_{\beta \in B} W_{i,\beta}^1 X_{\beta,\alpha} \tau_{\beta,\alpha}^2 \quad (3r_V^2 N_o) \quad (12455)$$

$$\tau_{\alpha,i}^3 = \sum_{\beta \in B} W_{i,\beta}^1 X_{\beta,\alpha} \tau_{\beta,\alpha}^2 \quad (3r_V^2 N_o) \quad (12468)$$

$$\tau_{i,a}^4 = \sum_{\alpha \in B} W_{a,\alpha}^4 \tau_{\alpha,i}^3 \quad (2r_V N_o N_v) \quad (12456)$$

$$\tau_{i,a}^4 = \sum_{\alpha \in B} W_{a,\alpha}^4 \tau_{\alpha,i}^3 \quad (2r_V N_o N_v) \quad (12469)$$

$$\tau_{\gamma,i}^5 = \sum_{a \in V} Y_{a,\gamma}^3 \tau_{i,a}^4 \quad (2r_T N_o N_v) \quad (12457)$$

$$\tau_{\gamma,i}^5 = \sum_{a \in V} Y_{a,\gamma}^1 \tau_{i,a}^4 \quad (2r_T N_o N_v) \quad (12470)$$

$$\tau_{\gamma,\delta,w}^6 = \sum_{i \in O} \tau_{\gamma,i}^5 \tau_{\delta,w,i}^0 \quad (2r_D r_T^2 N_o) \quad (12458)$$

$$\tau_{\gamma,\delta,w}^6 = \sum_{i \in O} \tau_{\gamma,i}^5 \tau_{\delta,w,i}^0 \quad (2r_D r_T^2 N_o) \quad (12471)$$

$$\tau_{\gamma,\delta,w}^7 = \sum_{a \in V} {}^2D_{a,w}^1 Y_{a,\gamma}^1 Y_{a,\delta}^{1,*} \quad (3r_D r_T^2 N_v) \quad (12459)$$

$$\tau_{\gamma,\delta,w}^7 = \sum_{a \in V} {}^2D_{a,w}^1 Y_{a,\gamma}^3 Y_{a,\delta}^{1,*} \quad (3r_D r_T^2 N_v) \quad (12472)$$

$$\tau_{\gamma,\delta,w}^8 = \sum_{i \in O} {}^2D_{i,w}^2 Y_{i,\gamma}^2 Y_{i,\delta}^{2,*} \quad (3r_D r_T^2 N_o) \quad (12460)$$

$$\tau_{\gamma,\delta,w}^8 = \sum_{i \in O} {}^2D_{i,w}^2 Y_{i,\gamma}^4 Y_{i,\delta}^{2,*} \quad (3r_D r_T^2 N_o) \quad (12473)$$

$$\tau_{\alpha,i,j}^7 = \sum_{\beta \in B} X_{\alpha,\beta} W_{j,\beta}^3 \tau_{\beta,i}^6 \quad (3r_V^2 N_o^2) \quad (12485)$$

$$\tau_{\gamma,\delta,w}^9 = \sum_{\epsilon \in A} Z_{\epsilon,\delta}^* \tau_{\gamma,\epsilon,w}^7 \tau_{\gamma,\epsilon,w}^8 \quad (3r_D r_T^3) \quad (12474)$$

$$\tau_{\gamma,\alpha,i}^8 = \sum_{j \in O} Y_{j,\gamma}^4 \tau_{\alpha,i,j}^7 \quad (2r_T r_V N_o^2) \quad (12486)$$

$$\tau_{\gamma,\delta,w}^{10} = \sum_{\epsilon \in A} Z_{\gamma,\epsilon} \tau_{\epsilon,\delta,w}^9 \quad (2r_D r_T^3) \quad (12475)$$

$$\tau_{\gamma,\delta,w,i}^9 = \sum_{\alpha \in B} \tau_{\gamma,\alpha,i}^8 \tau_{\gamma,\delta,\alpha,w}^5 \quad (2r_D r_T^2 r_V N_o) \quad (12487)$$

$${}^2R_{i,\gamma}^4 \leftarrow \sum_{\delta \in A} \sum_{w \in D} \frac{1}{2} {}^2D_{i,w}^4 Y_{i,\delta}^2 \tau_{\delta,\gamma,w}^{10} \tau_{\delta,\gamma,w}^6 \quad (4r_D r_T^2 N_o) \quad (12476)$$

$$\tau_{\gamma,\delta,i}^{10} = \sum_{\epsilon \in A} \sum_{w \in D} {}^2D_{i,w}^4 \tau_{\epsilon,\delta,w}^0 \tau_{\epsilon,\gamma,w,i}^9 \quad (3r_D r_T^3 N_o) \quad (12488)$$

Raw expression

$${}^2R_{j,\zeta}^4 \leftarrow - \sum_{\gamma \in A} \sum_{i \in O} \sum_{k \in O} \sum_{l \in O} \sum_{a \in V} \sum_{b \in V} \sum_{c \in V} \sum_{d \in V} {}^1T_{b,k} {}^1T_{c,l} Y_{a,\gamma}^{1,*} Y_{i,\gamma}^{2,*} Z_{\gamma,\zeta}^* Y_{b,\zeta}^{3,*} {}^2D_{a,i,b,j} {}^2T_{a,i,d,j} V_{k,d,l,c} \quad (12477)$$

$${}^2R_{i,\gamma}^4 \leftarrow \sum_{\delta \in A} \frac{1}{2} Z_{\delta,\gamma}^* \tau_{\delta,\gamma,i}^{10} \quad (2r_T^2 N_o) \quad (12489)$$

Raw expression

$${}^2R_{j,\zeta}^4 \leftarrow - \sum_{\gamma \in A} \sum_{i \in O} \sum_{k \in O} \sum_{l \in O} \sum_{a \in V} \sum_{b \in V} \sum_{c \in V} \sum_{d \in V} {}^1T_{b,k} {}^1T_{c,l} Y_{a,\gamma}^{1,*} Y_{i,\gamma}^{2,*} Z_{\gamma,\zeta}^* Y_{b,\zeta}^{3,*} {}^2D_{a,i,b,j} {}^2T_{d,j,a,i} V_{k,d,l,c} \quad (12490)$$

Factorized expression

$$\tau_{\gamma,\delta,w}^0 = \sum_{a \in V} {}^2D_{a,w}^3 Y_{a,\gamma}^3 Y_{a,\delta}^{3,*} \quad (3r_D r_T^2 N_v) \quad (12478)$$

Factorized expression

$$\tau_{\gamma,\delta,w}^0 = \sum_{a \in V} {}^2D_{a,w}^3 Y_{a,\gamma}^1 Y_{a,\delta}^{3,*} \quad (3r_D r_T^2 N_v) \quad (12491)$$

$$\tau_{\gamma,\alpha,w}^2 = \sum_{i \in O} {}^2D_{i,w}^2 Y_{i,\gamma}^{2,*} \tau_{\alpha,i}^1 \quad (3r_D r_T r_V N_o) \quad (12480)$$

$$\tau_{\alpha,i}^1 = \sum_{a \in V} {}^1T_{a,i} W_{a,\alpha}^4 \quad (2r_V N_o N_v) \quad (12492)$$

$$\tau_{\gamma,\delta,w}^3 = \sum_{a \in V} {}^2D_{a,w}^1 Y_{a,\gamma}^1 Y_{a,\delta}^{1,*} \quad (3r_D r_T^2 N_v) \quad (12481)$$

$$\tau_{\gamma,\alpha,w}^2 = \sum_{i \in O} {}^2D_{i,w}^2 Y_{i,\gamma}^{2,*} \tau_{\alpha,i}^1 \quad (3r_D r_T r_V N_o) \quad (12493)$$

$$\tau_{\gamma,\delta,w,i}^4 = \sum_{\epsilon \in A} Y_{i,\epsilon}^2 Z_{\epsilon,\gamma} \tau_{\epsilon,\delta,w}^3 \quad (3r_D r_T^3 N_o) \quad (12482)$$

$$\tau_{\gamma,\delta,w}^3 = \sum_{a \in V} {}^2D_{a,w}^1 Y_{a,\gamma}^3 Y_{a,\delta}^{1,*} \quad (3r_D r_T^2 N_v) \quad (12494)$$

$$\tau_{\gamma,\delta,\alpha,w}^5 = \sum_{i \in O} W_{i,\alpha}^1 \tau_{\delta,\alpha,w}^2 \tau_{\gamma,\delta,w,i}^4 \quad (3r_D r_T^2 r_V N_o) \quad (12483)$$

$$\tau_{\gamma,\delta,w,i}^4 = \sum_{\epsilon \in A} Z_{\gamma,\epsilon} Y_{i,\epsilon}^4 \tau_{\epsilon,\delta,w}^3 \quad (3r_D r_T^3 N_o) \quad (12495)$$

$$\tau_{\alpha,i}^6 = \sum_{a \in V} {}^1T_{a,i} W_{a,\alpha}^4 \quad (2r_V N_o N_v) \quad (12484)$$

$$\tau_{\gamma,\delta,\alpha,w}^5 = \sum_{i \in O} W_{i,\alpha}^3 \tau_{\delta,\alpha,w}^2 \tau_{\gamma,\delta,w,i}^4 \quad (3r_D r_T^2 r_V N_o) \quad (12496)$$

$$\tau^6_{\alpha,i} = \sum_{a \in V} {}^1T_{a,i} W^2_{a,\alpha} \quad (2r_V N_o N_v) \quad (12497)$$

$$\tau^5_{i,a} = \sum_{\alpha \in B} W^2_{a,\alpha} \tau^4_{\alpha,i} \quad (2r_V N_o N_v) \quad (12509)$$

$$\tau^7_{\alpha,i,j} = \sum_{\beta \in B} W^1_{j,\beta} X_{\beta,\alpha} \tau^6_{\beta,i} \quad (3r_V^2 N_o^2) \quad (12498)$$

$$\tau^6_{i,j} = \sum_{a \in V} {}^1T_{a,i} \tau^5_{j,a} \quad (2N_o^2 N_v) \quad (12510)$$

$$\tau^8_{\gamma,\alpha,i} = \sum_{j \in O} Y^2_{j,\gamma} \tau^7_{\alpha,i,j} \quad (2r_T r_V N_o^2) \quad (12499)$$

$$\tau^7_{\gamma,i} = \sum_{j \in O} Y^2_{j,\gamma} \tau^6_{i,j} \quad (2r_T N_o^2) \quad (12511)$$

$$\tau^9_{\gamma,\delta,w,i} = \sum_{\alpha \in B} \tau^8_{\gamma,\alpha,i} \tau^5_{\gamma,\delta,\alpha,w} \quad (2r_D r_T^2 r_V N_o) \quad (12500)$$

$$\tau^8_{\gamma,\delta,w} = \sum_{i \in O} {}^2D^2_{i,w} Y^{2,*}_{i,\delta} \tau^7_{\gamma,i} \quad (3r_D r_T^2 N_o) \quad (12512)$$

$$\tau^{10}_{\gamma,\delta,i} = \sum_{\epsilon \in A} \sum_{w \in D} {}^2D^4_{i,w} \tau^0_{\epsilon,\delta,w} \tau^9_{\epsilon,\gamma,w,i} \quad (3r_D r_T^3 N_o) \quad (12501)$$

$$\tau^9_{\gamma,\delta,w} = \sum_{\epsilon \in A} Z^*_{\epsilon,\delta} \tau^1_{\gamma,\epsilon,w} \tau^8_{\gamma,\epsilon,w} \quad (3r_D r_T^3) \quad (12513)$$

$${}^2R^4_{i,\gamma} \leftarrow \sum_{\delta \in A} \frac{1}{2} Z^*_{\delta,\gamma} \tau^{10}_{\delta,\gamma,i} \quad (2r_T^2 N_o) \quad (12502)$$

$$\tau^{10}_{\gamma,\delta,w} = \sum_{\epsilon \in A} Z_{\epsilon,\gamma} \tau^9_{\epsilon,\delta,w} \quad (2r_D r_T^3) \quad (12514)$$

Raw expression

$${}^2R^4_{i,\gamma} \leftarrow \sum_{\delta \in A} \sum_{w \in D} \frac{1}{2} {}^2D^4_{i,w} Y^4_{i,\delta} \tau^0_{\delta,\gamma,w} \tau^{10}_{\delta,\gamma,w} \quad (4r_D r_T^2 N_o) \quad (12515)$$

$$\begin{aligned} {}^2R^4_{j,\zeta} \leftarrow & - \sum_{\gamma \in A} \sum_{i \in O} \sum_{k \in O} \sum_{l \in O} \sum_{a \in V} \sum_{b \in V} \sum_{c \in V} \sum_{d \in V} {}^1T_{c,i} \\ & {}^1T_{d,k} Y^{1,*}_{a,\gamma} Y^{2,*}_{i,\gamma} Z^*_{\gamma,\zeta} \\ & Y^{3,*}_{b,\zeta} {}^2D^{a,i,b,j} {}^2T_{a,l,b,j} V_{k,d,l,c} \end{aligned} \quad (12503)$$

Raw expression

$$\begin{aligned} {}^2R^4_{j,\zeta} \leftarrow & - \sum_{\gamma \in A} \sum_{i \in O} \sum_{k \in O} \sum_{l \in O} \sum_{a \in V} \sum_{b \in V} \sum_{c \in V} \sum_{d \in V} {}^1T_{c,i} \\ & {}^1T_{d,k} Y^{1,*}_{a,\gamma} Y^{2,*}_{i,\gamma} Z^*_{\gamma,\zeta} \\ & Y^{3,*}_{b,\zeta} {}^2D^{a,i,b,j} {}^2T_{b,j,a,l} V_{k,d,l,c} \end{aligned} \quad (12516)$$

Factorized expression

Factorized expression

$$\tau^0_{\gamma,\delta,w} = \sum_{a \in V} {}^2D^3_{a,w} Y^3_{a,\gamma} Y^{3,*}_{a,\delta} \quad (3r_D r_T^2 N_v) \quad (12504)$$

$$\tau^0_{\gamma,\delta,w} = \sum_{a \in V} {}^2D^3_{a,w} Y^1_{a,\gamma} Y^{3,*}_{a,\delta} \quad (3r_D r_T^2 N_v) \quad (12517)$$

$$\tau^1_{\gamma,\delta,w} = \sum_{a \in V} {}^2D^1_{a,w} Y^1_{a,\gamma} Y^{1,*}_{a,\delta} \quad (3r_D r_T^2 N_v) \quad (12505)$$

$$\tau^1_{\gamma,\delta,w} = \sum_{a \in V} {}^2D^1_{a,w} Y^3_{a,\gamma} Y^{1,*}_{a,\delta} \quad (3r_D r_T^2 N_v) \quad (12518)$$

$$\tau^2_{\alpha,i} = \sum_{a \in V} {}^1T_{a,i} W^4_{a,\alpha} \quad (2r_V N_o N_v) \quad (12506)$$

$$\tau^2_{\alpha,i} = \sum_{a \in V} {}^1T_{a,i} W^4_{a,\alpha} \quad (2r_V N_o N_v) \quad (12519)$$

$$\tau^3_{\alpha,\beta} = \sum_{i \in O} W^1_{i,\alpha} \tau^2_{\beta,i} \quad (2r_V^2 N_o) \quad (12507)$$

$$\tau^3_{\alpha,\beta} = \sum_{i \in O} W^1_{i,\alpha} \tau^2_{\beta,i} \quad (2r_V^2 N_o) \quad (12520)$$

$$\tau^4_{\alpha,i} = \sum_{\beta \in B} X_{\alpha,\beta} W^3_{i,\beta} \tau^3_{\alpha,\beta} \quad (3r_V^2 N_o) \quad (12508)$$

$$\tau^4_{\alpha,i} = \sum_{\beta \in B} X_{\alpha,\beta} W^3_{i,\beta} \tau^3_{\alpha,\beta} \quad (3r_V^2 N_o) \quad (12521)$$

$$\tau^3_{\gamma,\delta,w} = \sum_{\epsilon \in A} Z^*_{\epsilon,\delta} \tau^1_{\gamma,\epsilon,w} \tau^2_{\gamma,\epsilon,w} \quad (3r_D r_T^3) \quad (12533)$$

$$\tau^5_{i,a} = \sum_{\alpha \in B} W^2_{a,\alpha} \tau^4_{\alpha,i} \quad (2r_V N_o N_v) \quad (12522)$$

$$\tau^4_{\gamma,\delta,w} = \sum_{\epsilon \in A} Z_{\epsilon,\gamma} \tau^3_{\epsilon,\delta,w} \quad (2r_D r_T^3) \quad (12534)$$

$$\tau^6_{i,j} = \sum_{a \in V} {}^1T_{a,i} \tau^5_{j,a} \quad (2N_o^2 N_v) \quad (12523)$$

$$\tau^5_{\alpha,i} = \sum_{a \in V} {}^1T_{a,i} W^4_{a,\alpha} \quad (2r_V N_o N_v) \quad (12535)$$

$$\tau^7_{\gamma,i} = \sum_{j \in O} Y^4_{j,\gamma} \tau^6_{i,j} \quad (2r_T N_o^2) \quad (12524)$$

$$\tau^6_{\alpha,\beta} = \sum_{i \in O} W^1_{i,\alpha} \tau^5_{\beta,i} \quad (2r_V^2 N_o) \quad (12536)$$

$$\tau^8_{\gamma,\delta,w} = \sum_{i \in O} {}^2D^2_{i,w} Y^{2,*}_{i,\delta} \tau^7_{\gamma,i} \quad (3r_D r_T^2 N_o) \quad (12525)$$

$$\tau^7_{\alpha,i} = \sum_{\beta \in B} X_{\alpha,\beta} W^3_{i,\beta} \tau^6_{\alpha,\beta} \quad (3r_V^2 N_o) \quad (12537)$$

$$\tau^9_{\gamma,\delta,w} = \sum_{\epsilon \in A} Z^*_{\epsilon,\delta} \tau^1_{\gamma,\epsilon,w} \tau^8_{\gamma,\epsilon,w} \quad (3r_D r_T^3) \quad (12526)$$

$$\tau^8_{i,a} = \sum_{\alpha \in B} W^2_{a,\alpha} \tau^7_{\alpha,i} \quad (2r_V N_o N_v) \quad (12538)$$

$$\tau^{10}_{\gamma,\delta,w} = \sum_{\epsilon \in A} Z_{\gamma,\epsilon} \tau^9_{\epsilon,\delta,w} \quad (2r_D r_T^3) \quad (12527)$$

$$\tau^9_{i,j} = \sum_{a \in V} {}^1T_{a,i} \tau^8_{j,a} \quad (2N_o^2 N_v) \quad (12539)$$

$${}^2R^4_{i,\gamma} \leftarrow \sum_{\delta \in A} \sum_{w \in D} \frac{1}{2} {}^2D^4_{i,w} Y^2_{i,\delta} \tau^0_{\delta,\gamma,w} \tau^{10}_{\delta,\gamma,w} \quad (4r_D r_T^2 N_o) \quad (12528)$$

$$\tau^{10}_{\gamma,i} = \sum_{j \in O} Y^4_{j,\gamma} \tau^9_{i,j} \quad (2r_T N_o^2) \quad (12540)$$

Raw expression

$${}^2R^4_{j,\zeta} \leftarrow - \sum_{\gamma \in A} \sum_{i \in O} \sum_{k \in O} \sum_{l \in O} \sum_{a \in V} \sum_{b \in V} \sum_{c \in V} \sum_{d \in V} {}^1T_{c,k} \quad (12529)$$

$${}^1T_{d,j} Y^{1,*}_{a,\gamma} Y^{2,*}_{i,\gamma} Z^*_{\gamma,\zeta} Y^{3,*}_{b,\zeta} {}^2D^{a,i,b,j}_{a,i,b,l} V_{k,c,l,d}$$

Factorized expression

$$\tau^0_{\gamma,\delta,w} = \sum_{a \in V} {}^2D^3_{a,w} Y^3_{a,\gamma} Y^{3,*}_{a,\delta} \quad (3r_D r_T^2 N_v) \quad (12530)$$

$$\tau^1_{\gamma,\delta,w} = \sum_{a \in V} {}^2D^1_{a,w} Y^1_{a,\gamma} Y^{1,*}_{a,\delta} \quad (3r_D r_T^2 N_v) \quad (12531)$$

$$\tau^2_{\gamma,\delta,w} = \sum_{i \in O} {}^2D^2_{i,w} Y^2_{i,\gamma} Y^{2,*}_{i,\delta} \quad (3r_D r_T^2 N_o) \quad (12532)$$

$${}^2R^4_{i,\gamma} \leftarrow \sum_{\delta \in A} \sum_{w \in D} \frac{1}{2} {}^2D^4_{i,w} \tau^{10}_{\delta,i} \tau^0_{\delta,\gamma,w} \tau^4_{\delta,\gamma,w} \quad (4r_D r_T^2 N_o) \quad (12541)$$

Raw expression

$${}^2R^4_{j,\zeta} \leftarrow - \sum_{\gamma \in A} \sum_{i \in O} \sum_{k \in O} \sum_{l \in O} \sum_{a \in V} \sum_{b \in V} \sum_{c \in V} \sum_{d \in V} {}^1T_{c,k} \quad (12542)$$

$${}^1T_{d,j} Y^{1,*}_{a,\gamma} Y^{2,*}_{i,\gamma} Z^*_{\gamma,\zeta} Y^{3,*}_{b,\zeta} {}^2D^{a,i,b,j}_{b,l,a,i} V_{k,c,l,d}$$

Factorized expression

$$\tau^0_{\gamma,\delta,w} = \sum_{a \in V} {}^2D^3_{a,w} Y^1_{a,\gamma} Y^{3,*}_{a,\delta} \quad (3r_D r_T^2 N_v) \quad (12543)$$

$$\tau^1_{\gamma,\delta,w} = \sum_{a \in V} {}^2D^1_{a,w} Y^3_{a,\gamma} Y^{1,*}_{a,\delta} \quad (3r_D r_T^2 N_v) \quad (12544)$$

$$\tau_{\gamma,\delta,w}^2 = \sum_{i \in O} {}^2D_{i,w}^2 Y_{i,\gamma}^4 Y_{i,\delta}^{2,*} \quad (3r_D r_T^2 N_o) \quad (12545)$$

$$\tau_{\gamma,\delta,w}^1 = \sum_{i \in O} {}^2D_{i,w}^2 Y_{i,\gamma}^2 Y_{i,\delta}^{2,*} \quad (3r_D r_T^2 N_o) \quad (12557)$$

$$\tau_{\gamma,\delta,w}^3 = \sum_{\epsilon \in A} Z_{\epsilon,\delta}^* \tau_{\gamma,\epsilon,w}^1 \tau_{\gamma,\epsilon,w}^2 \quad (3r_D r_T^3) \quad (12546)$$

$$\tau_{\gamma,\delta,w}^2 = \sum_{\epsilon \in A} Z_{\epsilon,\delta}^* \tau_{\gamma,\epsilon,w}^0 \tau_{\gamma,\epsilon,w}^1 \quad (3r_D r_T^3) \quad (12558)$$

$$\tau_{\gamma,\delta,w}^4 = \sum_{\epsilon \in A} Z_{\gamma,\epsilon} \tau_{\epsilon,\delta,w}^3 \quad (2r_D r_T^3) \quad (12547)$$

$$\tau_{\gamma,\alpha}^3 = \sum_{a \in V} W_{a,\alpha}^4 Y_{a,\gamma}^3 \quad (2r_T r_V N_v) \quad (12559)$$

$$\tau_{\alpha,i}^5 = \sum_{a \in V} {}^1T_{a,i} W_{a,\alpha}^4 \quad (2r_V N_o N_v) \quad (12548)$$

$$\tau_{\gamma,\alpha}^4 = \sum_{i \in O} W_{i,\alpha}^3 Y_{i,\gamma}^4 \quad (2r_T r_V N_o) \quad (12560)$$

$$\tau_{\alpha,\beta}^6 = \sum_{i \in O} W_{i,\alpha}^1 \tau_{\beta,i}^5 \quad (2r_V^2 N_o) \quad (12549)$$

$$\tau_{\gamma,\alpha}^5 = \sum_{\beta \in B} X_{\alpha,\beta} \tau_{\gamma,\beta}^3 \tau_{\gamma,\beta}^4 \quad (3r_T r_V^2) \quad (12561)$$

$$\tau_{\alpha,i}^7 = \sum_{\beta \in B} X_{\alpha,\beta} W_{i,\beta}^3 \tau_{\alpha,\beta}^6 \quad (3r_V^2 N_o) \quad (12550)$$

$$\tau_{\gamma,\alpha}^6 = \sum_{a \in V} W_{a,\alpha}^2 Y_{a,\gamma}^3 \quad (2r_T r_V N_v) \quad (12562)$$

$$\tau_{i,a}^8 = \sum_{\alpha \in B} W_{a,\alpha}^2 \tau_{\alpha,i}^7 \quad (2r_V N_o N_v) \quad (12551)$$

$$\tau_{\gamma,\alpha}^7 = \sum_{i \in O} W_{i,\alpha}^1 Y_{i,\gamma}^4 \quad (2r_T r_V N_o) \quad (12563)$$

$$\tau_{i,j}^9 = \sum_{a \in V} {}^1T_{a,i} \tau_{j,a}^8 \quad (2N_o^2 N_v) \quad (12552)$$

$$\tau_{\gamma,\delta}^8 = \sum_{\alpha \in B} \tau_{\delta,\alpha}^5 \tau_{\gamma,\alpha}^6 \tau_{\gamma,\alpha}^7 \quad (3r_T^2 r_V) \quad (12564)$$

$$\tau_{\gamma,i}^{10} = \sum_{j \in O} Y_{j,\gamma}^2 \tau_{i,j}^9 \quad (2r_T N_o^2) \quad (12553)$$

$$\tau_{\gamma,\delta}^9 = \sum_{\epsilon \in A} Z_{\gamma,\epsilon} \tau_{\delta,\epsilon}^8 \quad (2r_T^3) \quad (12565)$$

$${}^2R_{i,\gamma}^4 \leftarrow \sum_{\delta \in A} \sum_{w \in D} \frac{1}{2} {}^2D_{i,w}^4 \tau_{\delta,i}^{10} \tau_{\delta,\gamma,w}^0 \tau_{\delta,\gamma,w}^4 \quad (4r_D r_T^2 N_o) \quad (12554)$$

$$\tau_{\gamma,\delta}^{10} = \sum_{\epsilon \in A} Z_{\gamma,\epsilon} \tau_{\delta,\epsilon}^9 \quad (2r_T^3) \quad (12566)$$

$$\tau_{\gamma,\delta,w}^{11} = \sum_{\epsilon \in A} \tau_{\epsilon,\gamma}^{10} \tau_{\epsilon,\delta,w}^2 \quad (2r_D r_T^3) \quad (12567)$$

### I. Contributions from $(H^2 T^2 T)_c$

Raw expression

$${}^2R_{j,\zeta}^4 \leftarrow \sum_{\gamma \in A} \sum_{i \in O} \sum_{k \in O} \sum_{l \in O} \sum_{a \in V} \sum_{b \in V} \sum_{c \in V} \sum_{d \in V} Y_{a,\gamma}^{1,*} Y_{i,\gamma}^{2,*} Z_{\gamma,\zeta}^* Y_{b,\zeta}^{3,*} {}^2D_{a,i,b,j} {}^2T_{a,i,c,k} {}^2T_{b,j,d,l} V_{k,c,l,d} \quad (12555)$$

Factorized expression

$$\tau_{\gamma,\delta,w}^0 = \sum_{a \in V} {}^2D_{a,w}^1 Y_{a,\gamma}^1 Y_{a,\delta}^{1,*} \quad (3r_D r_T^2 N_v) \quad (12556)$$

$$\tau_{\gamma,\delta,w}^{12} = \sum_{a \in V} {}^2D_{a,w}^3 Y_{a,\gamma}^1 Y_{a,\delta}^{3,*} \quad (3r_D r_T^2 N_v) \quad (12568)$$

$${}^2R_{i,\gamma}^4 \leftarrow \sum_{\delta \in A} \sum_{w \in D} {}^2D_{i,w}^4 Y_{i,\delta}^2 \tau_{\delta,\gamma,w}^{11} \tau_{\delta,\gamma,w}^{12} \quad (4r_D r_T^2 N_o) \quad (12569)$$

Raw expression

$${}^2R_{j,\zeta}^4 \leftarrow \sum_{\gamma \in A} \sum_{i \in O} \sum_{k \in O} \sum_{l \in O} \sum_{a \in V} \sum_{b \in V} \sum_{c \in V} \sum_{d \in V} Y_{a,\gamma}^{1,*} Y_{i,\gamma}^{2,*} Z_{\gamma,\zeta}^* Y_{b,\zeta}^{3,*} {}^2D_{a,i,b,j} {}^2T_{a,i,c,k} {}^2T_{d,l,b,j} V_{k,c,l,d} \quad (12570)$$



Factorized expression

$$\tau^0_{\gamma,\delta,w} = \sum_{a \in V} {}^2D^1_{a,w} Y^1_{a,\gamma} Y^{1,*}_{a,\delta} \quad (3r_D r_T^2 N_v) \quad (12571)$$

$$\tau^1_{\gamma,\delta,w} = \sum_{i \in O} {}^2D^2_{i,w} Y^2_{i,\gamma} Y^{2,*}_{i,\delta} \quad (3r_D r_T^2 N_o) \quad (12572)$$

$$\tau^2_{\gamma,\delta,w} = \sum_{\epsilon \in A} Z^*_{\epsilon,\delta} \tau^0_{\gamma,\epsilon,w} \tau^1_{\gamma,\epsilon,w} \quad (3r_D r_T^3) \quad (12573)$$

$$\tau^3_{\gamma,\alpha} = \sum_{a \in V} W^2_{a,\alpha} Y^3_{a,\gamma} \quad (2r_T r_V N_v) \quad (12574)$$

$$\tau^4_{\gamma,\alpha} = \sum_{i \in O} W^1_{i,\alpha} Y^4_{i,\gamma} \quad (2r_T r_V N_o) \quad (12575)$$

$$\tau^5_{\gamma,\alpha} = \sum_{a \in V} W^4_{a,\alpha} Y^1_{a,\gamma} \quad (2r_T r_V N_v) \quad (12576)$$

$$\tau^6_{\gamma,\alpha} = \sum_{i \in O} W^3_{i,\alpha} Y^2_{i,\gamma} \quad (2r_T r_V N_o) \quad (12577)$$

$$\tau^7_{\gamma,\alpha} = \sum_{\beta \in B} X_{\alpha,\beta} \tau^5_{\gamma,\beta} \tau^6_{\gamma,\beta} \quad (3r_T r_V^2) \quad (12578)$$

$$\tau^8_{\gamma,\delta} = \sum_{\alpha \in B} \tau^3_{\delta,\alpha} \tau^4_{\delta,\alpha} \tau^7_{\gamma,\alpha} \quad (3r_T^2 r_V) \quad (12579)$$

$$\tau^9_{\gamma,\delta} = \sum_{\epsilon \in A} Z_{\delta,\epsilon} \tau^8_{\gamma,\epsilon} \quad (2r_T^3) \quad (12580)$$

$$\tau^{10}_{\gamma,\delta} = \sum_{\epsilon \in A} Z_{\epsilon,\delta} \tau^9_{\epsilon,\gamma} \quad (2r_T^3) \quad (12581)$$

$$\tau^{11}_{\gamma,\delta,w} = \sum_{\epsilon \in A} \tau^{10}_{\epsilon,\gamma} \tau^2_{\epsilon,\delta,w} \quad (2r_D r_T^3) \quad (12582)$$

$$\tau^{12}_{\gamma,\delta,w} = \sum_{a \in V} {}^2D^3_{a,w} Y^3_{a,\gamma} Y^{3,*}_{a,\delta} \quad (3r_D r_T^2 N_v) \quad (12583)$$

$${}^2R^4_{i,\gamma} \leftarrow \sum_{\delta \in A} \sum_{w \in D} {}^2D^4_{i,w} Y^4_{i,\delta} \tau^{11}_{\delta,\gamma,w} \tau^{12}_{\delta,\gamma,w} \quad (4r_D r_T^2 N_o) \quad (12584)$$

Raw expression

$${}^2R^4_{j,\zeta} \leftarrow \sum_{\gamma \in A} \sum_{i \in O} \sum_{k \in O} \sum_{l \in O} \sum_{a \in V} \sum_{b \in V} \sum_{c \in V} \sum_{d \in V} Y^{1,*}_{a,\gamma} Y^{2,*}_{i,\gamma} Z^*_{\gamma,\zeta} Y^{3,*}_{b,\zeta} {}^2D^{a,i,b,j} {}^2T_{b,j,d,l} {}^2T_{c,k,a,i} V_{k,c,l,d} \quad (12585)$$

Factorized expression

$$\tau^0_{\gamma,\delta,w} = \sum_{a \in V} {}^2D^1_{a,w} Y^3_{a,\gamma} Y^{1,*}_{a,\delta} \quad (3r_D r_T^2 N_v) \quad (12586)$$

$$\tau^1_{\gamma,\delta,w} = \sum_{i \in O} {}^2D^2_{i,w} Y^4_{i,\gamma} Y^{2,*}_{i,\delta} \quad (3r_D r_T^2 N_o) \quad (12587)$$

$$\tau^2_{\gamma,\delta,w} = \sum_{\epsilon \in A} Z^*_{\epsilon,\delta} \tau^0_{\gamma,\epsilon,w} \tau^1_{\gamma,\epsilon,w} \quad (3r_D r_T^3) \quad (12588)$$

$$\tau^3_{\gamma,\alpha} = \sum_{a \in V} W^4_{a,\alpha} Y^3_{a,\gamma} \quad (2r_T r_V N_v) \quad (12589)$$

$$\tau^4_{\gamma,\alpha} = \sum_{i \in O} W^3_{i,\alpha} Y^4_{i,\gamma} \quad (2r_T r_V N_o) \quad (12590)$$

$$\tau^5_{\gamma,\alpha} = \sum_{\beta \in B} X_{\alpha,\beta} \tau^3_{\gamma,\beta} \tau^4_{\gamma,\beta} \quad (3r_T r_V^2) \quad (12591)$$

$$\tau^6_{\gamma,\alpha} = \sum_{a \in V} W^2_{a,\alpha} Y^1_{a,\gamma} \quad (2r_T r_V N_v) \quad (12592)$$

$$\tau^7_{\gamma,\alpha} = \sum_{i \in O} W^1_{i,\alpha} Y^2_{i,\gamma} \quad (2r_T r_V N_o) \quad (12593)$$

$$\tau^8_{\gamma,\delta} = \sum_{\alpha \in B} \tau^5_{\delta,\alpha} \tau^6_{\gamma,\alpha} \tau^7_{\gamma,\alpha} \quad (3r_T^2 r_V) \quad (12594)$$

$$\tau^9_{\gamma,\delta} = \sum_{\epsilon \in A} Z_{\delta,\epsilon} \tau^8_{\gamma,\epsilon} \quad (2r_T^3) \quad (12595)$$

$$\tau^{10}_{\gamma,\delta} = \sum_{\epsilon \in A} Z_{\epsilon,\delta} \tau^9_{\epsilon,\gamma} \quad (2r_T^3) \quad (12596)$$

$$\tau^{11}_{\gamma,\delta,w} = \sum_{\epsilon \in A} \tau^{10}_{\gamma,\epsilon} \tau^2_{\epsilon,\delta,w} \quad (2r_D r_T^3) \quad (12597)$$

$$\tau^{12}_{\gamma,\delta,w} = \sum_{a \in V} {}^2D^3_{a,w} Y^1_{a,\gamma} Y^{3,*}_{a,\delta} \quad (3r_D r_T^2 N_v) \quad (12598)$$

$$\tau^{10}_{\gamma,\delta} = \sum_{\epsilon \in A} Z_{\epsilon,\gamma} \tau^9_{\epsilon,\delta} \quad (2r_T^3) \quad (12611)$$

$${}^2R^4_{i,\gamma} \leftarrow \sum_{\delta \in A} \sum_{w \in D} {}^2D^4_{i,w} Y^2_{i,\delta} \tau^{11}_{\delta,\gamma,w} \tau^{12}_{\delta,\gamma,w} \quad (4r_D r_T^2 N_o) \quad (12599)$$

$$\tau^{11}_{\gamma,\delta,w} = \sum_{\epsilon \in A} \tau^{10}_{\epsilon,\gamma} \tau^2_{\epsilon,\delta,w} \quad (2r_D r_T^3) \quad (12612)$$

$$\tau^{12}_{\gamma,\delta,w} = \sum_{a \in V} {}^2D^3_{a,w} Y^3_{a,\gamma} Y^{3,*}_{a,\delta} \quad (3r_D r_T^2 N_v) \quad (12613)$$

Raw expression

$${}^2R^4_{j,\zeta} \leftarrow \sum_{\gamma \in A} \sum_{i \in O} \sum_{k \in O} \sum_{l \in O} \sum_{a \in V} \sum_{b \in V} \sum_{c \in V} \sum_{d \in V} Y^{1,*}_{a,\gamma} Y^{2,*}_{i,\gamma} Z^*_{\gamma,\zeta} Y^{3,*}_{b,\zeta} {}^2D^{a,i,b,j} {}^2T_{c,k,a,i} {}^2T_{d,l,b,j} V_{k,c,l,d} \quad (12600)$$

$${}^2R^4_{i,\gamma} \leftarrow \sum_{\delta \in A} \sum_{w \in D} {}^2D^4_{i,w} Y^4_{i,\delta} \tau^{11}_{\delta,\gamma,w} \tau^{12}_{\delta,\gamma,w} \quad (4r_D r_T^2 N_o) \quad (12614)$$

Factorized expression

$$\tau^0_{\gamma,\delta,w} = \sum_{a \in V} {}^2D^1_{a,w} Y^3_{a,\gamma} Y^{1,*}_{a,\delta} \quad (3r_D r_T^2 N_v) \quad (12601)$$

Raw expression

$${}^2R^4_{j,\zeta} \leftarrow - \sum_{\gamma \in A} \sum_{i \in O} \sum_{k \in O} \sum_{l \in O} \sum_{a \in V} \sum_{b \in V} \sum_{c \in V} \sum_{d \in V} \frac{1}{2} Y^{1,*}_{a,\gamma} Y^{2,*}_{i,\gamma} Z^*_{\gamma,\zeta} Y^{3,*}_{b,\zeta} {}^2D^{a,i,b,j} {}^2T_{a,i,b,k} {}^2T_{c,j,d,l} V_{k,c,l,d} \quad (12615)$$

$$\tau^1_{\gamma,\delta,w} = \sum_{i \in O} {}^2D^2_{i,w} Y^4_{i,\gamma} Y^{2,*}_{i,\delta} \quad (3r_D r_T^2 N_o) \quad (12602)$$

Factorized expression

$$\tau^2_{\gamma,\delta,w} = \sum_{\epsilon \in A} Z^*_{\epsilon,\delta} \tau^0_{\gamma,\epsilon,w} \tau^1_{\gamma,\epsilon,w} \quad (3r_D r_T^3) \quad (12603)$$

$$\tau^0_{\gamma,\delta,w} = \sum_{a \in V} {}^2D^1_{a,w} Y^1_{a,\gamma} Y^{1,*}_{a,\delta} \quad (3r_D r_T^2 N_v) \quad (12616)$$

$$\tau^3_{\gamma,\alpha} = \sum_{a \in V} W^4_{a,\alpha} Y^1_{a,\gamma} \quad (2r_T r_V N_v) \quad (12604)$$

$$\tau^1_{\gamma,\delta,w} = \sum_{i \in O} {}^2D^2_{i,w} Y^2_{i,\gamma} Y^{2,*}_{i,\delta} \quad (3r_D r_T^2 N_o) \quad (12617)$$

$$\tau^4_{\gamma,\alpha} = \sum_{i \in O} W^3_{i,\alpha} Y^2_{i,\gamma} \quad (2r_T r_V N_o) \quad (12605)$$

$$\tau^2_{\gamma,\delta,w} = \sum_{\epsilon \in A} Z^*_{\epsilon,\delta} \tau^0_{\gamma,\epsilon,w} \tau^1_{\gamma,\epsilon,w} \quad (3r_D r_T^3) \quad (12618)$$

$$\tau^5_{\gamma,\alpha} = \sum_{\beta \in B} X_{\alpha,\beta} \tau^3_{\gamma,\beta} \tau^4_{\gamma,\beta} \quad (3r_T r_V^2) \quad (12606)$$

$$\tau^3_{\gamma,\alpha} = \sum_{a \in V} W^2_{a,\alpha} Y^3_{a,\gamma} \quad (2r_T r_V N_v) \quad (12619)$$

$$\tau^6_{\gamma,\alpha} = \sum_{a \in V} W^2_{a,\alpha} Y^1_{a,\gamma} \quad (2r_T r_V N_v) \quad (12607)$$

$$\tau^4_{\gamma,\alpha,i} = \sum_{\beta \in B} W^1_{i,\beta} X_{\beta,\alpha} \tau^3_{\gamma,\beta} \quad (3r_T r_V^2 N_o) \quad (12620)$$

$$\tau^7_{\gamma,\alpha} = \sum_{i \in O} W^1_{i,\alpha} Y^2_{i,\gamma} \quad (2r_T r_V N_o) \quad (12608)$$

$$\tau^5_{\gamma,\alpha} = \sum_{i \in O} W^3_{i,\alpha} Y^4_{i,\gamma} \quad (2r_T r_V N_o) \quad (12621)$$

$$\tau^8_{\gamma,\delta} = \sum_{\alpha \in B} \tau^5_{\delta,\alpha} \tau^6_{\gamma,\alpha} \tau^7_{\gamma,\alpha} \quad (3r_T^2 r_V) \quad (12609)$$

$$\tau^6_{\gamma,\alpha} = \sum_{a \in V} W^4_{a,\alpha} Y^3_{a,\gamma} \quad (2r_T r_V N_v) \quad (12622)$$

$$\tau^9_{\gamma,\delta} = \sum_{\epsilon \in A} Z_{\epsilon,\delta} \tau^8_{\gamma,\epsilon} \quad (2r_T^3) \quad (12610)$$

$$\tau^7_{\gamma,\delta,i} = \sum_{\alpha \in B} \tau^5_{\gamma,\alpha} \tau^6_{\delta,\alpha} \tau^4_{\gamma,\alpha,i} \quad (3r_T^2 r_V N_o) \quad (12623)$$

$$\tau_{\gamma,\delta}^8 = \sum_{i \in O} Y_{i,\delta}^4 \tau_{\gamma,\delta,i}^7 \quad (2r_T^2 N_o) \quad (12624)$$

$$\tau_{\gamma,\alpha}^6 = \sum_{i \in O} W_{i,\alpha}^3 Y_{i,\gamma}^4 \quad (2r_T r_V N_o) \quad (12637)$$

$$\tau_{\gamma,\delta}^9 = \sum_{\epsilon \in A} Z_{\gamma,\epsilon} \tau_{\delta,\epsilon}^8 \quad (2r_T^3) \quad (12625)$$

$$\tau_{\gamma,\alpha}^7 = \sum_{\beta \in B} X_{\alpha,\beta} \tau_{\gamma,\beta}^5 \tau_{\gamma,\beta}^6 \quad (3r_T r_V^2) \quad (12638)$$

$$\tau_{\gamma,\delta}^{10} = \sum_{\epsilon \in A} Z_{\gamma,\epsilon} \tau_{\delta,\epsilon}^9 \quad (2r_T^3) \quad (12626)$$

$$\tau_{\gamma,\alpha}^8 = \sum_{\delta \in A} Z_{\gamma,\delta} \tau_{\delta,\alpha}^7 \quad (2r_T^2 r_V) \quad (12639)$$

$$\tau_{\gamma,\delta,w}^{11} = \sum_{\epsilon \in A} \tau_{\gamma,\epsilon}^{10} \tau_{\epsilon,\delta,w}^2 \quad (2r_D r_T^3) \quad (12627)$$

$$\tau_{\gamma,a}^9 = \sum_{\alpha \in B} W_{a,\alpha}^2 \tau_{\gamma,\alpha}^4 \tau_{\gamma,\alpha}^8 \quad (3r_T r_V N_v) \quad (12640)$$

$$\tau_{\gamma,\delta,w}^{12} = \sum_{a \in V} {}^2D_{a,w}^3 Y_{a,\gamma}^1 Y_{a,\delta}^{3,*} \quad (3r_D r_T^2 N_v) \quad (12628)$$

$$\tau_{a,b}^{10} = \sum_{\gamma \in A} Y_{b,\gamma}^1 \tau_{\gamma,a}^9 \quad (2r_T N_v^2) \quad (12641)$$

$${}^2R_{i,\gamma}^4 \leftarrow - \sum_{\delta \in A} \sum_{w \in D} \frac{1}{2} {}^2D_{i,w}^4 Y_{i,\delta}^2 \tau_{\delta,\gamma,w}^{11} \tau_{\delta,\gamma,w}^{12} \quad (4r_D r_T^2 N_o) \quad (12629)$$

$$\tau_{\gamma,a}^{11} = \sum_{b \in V} Y_{b,\gamma}^3 \tau_{b,a}^{10} \quad (2r_T N_v^2) \quad (12642)$$

$$\tau_{\gamma,\delta,w}^{12} = \sum_{a \in V} {}^2D_{a,w}^3 Y_{a,\delta}^{3,*} \tau_{\gamma,a}^{11} \quad (3r_D r_T^2 N_v) \quad (12643)$$

Raw expression

$${}^2R_{j,\zeta}^4 \leftarrow - \sum_{\gamma \in A} \sum_{i \in O} \sum_{k \in O} \sum_{l \in O} \sum_{a \in V} \sum_{b \in V} \sum_{c \in V} \sum_{d \in V} \frac{1}{2} Y_{a,\gamma}^{1,*} Y_{i,\gamma}^{2,*} Z_{\gamma,\zeta}^* Y_{b,\zeta}^{3,*} {}^2D_{a,i,b,j}^a {}^2T_{a,i,b,k} {}^2T_{c,l,d,j} V_{k,d,l,c} \quad (12630)$$

$${}^2R_{i,\gamma}^4 \leftarrow - \sum_{\delta \in A} \sum_{w \in D} \frac{1}{2} {}^2D_{i,w}^4 Y_{i,\delta}^4 \tau_{\delta,\gamma,w}^{12} \tau_{\delta,\gamma,w}^3 \quad (4r_D r_T^2 N_o) \quad (12644)$$

Factorized expression

$$\tau_{\gamma,\delta,w}^0 = \sum_{a \in V} {}^2D_{a,w}^1 Y_{a,\gamma}^1 Y_{a,\delta}^{1,*} \quad (3r_D r_T^2 N_v) \quad (12631)$$

Raw expression

$${}^2R_{j,\zeta}^4 \leftarrow - \sum_{\gamma \in A} \sum_{i \in O} \sum_{k \in O} \sum_{l \in O} \sum_{a \in V} \sum_{b \in V} \sum_{c \in V} \sum_{d \in V} \frac{1}{2} Y_{a,\gamma}^{1,*} Y_{i,\gamma}^{2,*} Z_{\gamma,\zeta}^* Y_{b,\zeta}^{3,*} {}^2D_{a,i,b,j}^a {}^2T_{a,i,c,k} {}^2T_{b,j,d,l} V_{k,d,l,c} \quad (12645)$$

$$\tau_{\gamma,\delta,w}^1 = \sum_{i \in O} {}^2D_{i,w}^2 Y_{i,\gamma}^2 Y_{i,\delta}^{2,*} \quad (3r_D r_T^2 N_o) \quad (12632)$$

Factorized expression

$$\tau_{\gamma,\delta,w}^2 = \sum_{\epsilon \in A} Z_{\epsilon,\delta}^* \tau_{\gamma,\epsilon,w}^0 \tau_{\gamma,\epsilon,w}^1 \quad (3r_D r_T^3) \quad (12633)$$

$$\tau_{\gamma,\delta,w}^0 = \sum_{a \in V} {}^2D_{a,w}^1 Y_{a,\gamma}^1 Y_{a,\delta}^{1,*} \quad (3r_D r_T^2 N_v) \quad (12646)$$

$$\tau_{\gamma,\delta,w}^3 = \sum_{\epsilon \in A} Z_{\epsilon,\gamma} \tau_{\epsilon,\delta,w}^2 \quad (2r_D r_T^3) \quad (12634)$$

$$\tau_{\gamma,\delta,w}^1 = \sum_{i \in O} {}^2D_{i,w}^2 Y_{i,\gamma}^2 Y_{i,\delta}^{2,*} \quad (3r_D r_T^2 N_o) \quad (12647)$$

$$\tau_{\gamma,\alpha}^4 = \sum_{i \in O} W_{i,\alpha}^1 Y_{i,\gamma}^2 \quad (2r_T r_V N_o) \quad (12635)$$

$$\tau_{\gamma,\delta,w}^2 = \sum_{\epsilon \in A} Z_{\epsilon,\delta}^* \tau_{\gamma,\epsilon,w}^0 \tau_{\gamma,\epsilon,w}^1 \quad (3r_D r_T^3) \quad (12648)$$

$$\tau_{\gamma,\alpha}^5 = \sum_{a \in V} W_{a,\alpha}^4 Y_{a,\gamma}^3 \quad (2r_T r_V N_v) \quad (12636)$$

$$\tau_{\gamma,\alpha}^3 = \sum_{a \in V} W_{a,\alpha}^2 Y_{a,\gamma}^3 \quad (2r_T r_V N_v) \quad (12649)$$

$$\tau^4_{\gamma,\alpha} = \sum_{i \in O} W^1_{i,\alpha} Y^4_{i,\gamma} \quad (2r_T r_V N_o) \quad (12650)$$

$$\tau^1_{\gamma,\alpha} = \sum_{i \in O} W^1_{i,\alpha} Y^2_{i,\gamma} \quad (2r_T r_V N_o) \quad (12663)$$

$$\tau^5_{\gamma,\alpha} = \sum_{\beta \in B} X_{\beta,\alpha} \tau^3_{\gamma,\beta} \tau^4_{\gamma,\beta} \quad (3r_T r_V^2) \quad (12651)$$

$$\tau^2_{\gamma,\alpha} = \sum_{a \in V} W^4_{a,\alpha} Y^3_{a,\gamma} \quad (2r_T r_V N_v) \quad (12664)$$

$$\tau^6_{\gamma,\alpha} = \sum_{\delta \in A} Z_{\gamma,\delta} \tau^5_{\delta,\alpha} \quad (2r_T^2 r_V) \quad (12652)$$

$$\tau^3_{\gamma,\alpha} = \sum_{i \in O} W^3_{i,\alpha} Y^4_{i,\gamma} \quad (2r_T r_V N_o) \quad (12665)$$

$$\tau^7_{\gamma,\alpha} = \sum_{a \in V} W^4_{a,\alpha} Y^3_{a,\gamma} \quad (2r_T r_V N_v) \quad (12653)$$

$$\tau^4_{\gamma,\alpha} = \sum_{\beta \in B} X_{\alpha,\beta} \tau^2_{\gamma,\beta} \tau^3_{\gamma,\beta} \quad (3r_T r_V^2) \quad (12666)$$

$$\tau^8_{\gamma,\delta,i} = \sum_{\alpha \in B} W^3_{i,\alpha} \tau^6_{\gamma,\alpha} \tau^7_{\delta,\alpha} \quad (3r_T^2 r_V N_o) \quad (12654)$$

$$\tau^5_{\gamma,\alpha} = \sum_{\delta \in A} Z_{\gamma,\delta} \tau^4_{\delta,\alpha} \quad (2r_T^2 r_V) \quad (12667)$$

$$\tau^9_{\gamma,\delta,\epsilon} = \sum_{i \in O} Y^2_{i,\gamma} \tau^8_{\delta,\epsilon,i} \quad (2r_T^3 N_o) \quad (12655)$$

$$\tau^6_{\gamma,a} = \sum_{\alpha \in B} W^2_{a,\alpha} \tau^1_{\gamma,\alpha} \tau^5_{\gamma,\alpha} \quad (3r_T r_V N_v) \quad (12668)$$

$$\tau^{10}_{\gamma,\delta,i} = \sum_{\epsilon \in A} Z_{\gamma,\epsilon} Y^4_{i,\epsilon} \tau^9_{\gamma,\delta,\epsilon} \quad (3r_T^3 N_o) \quad (12656)$$

$$\tau^7_{a,b} = \sum_{\gamma \in A} Y^1_{b,\gamma} \tau^6_{\gamma,a} \quad (2r_T N_v^2) \quad (12669)$$

$$\tau^{11}_{\gamma,\delta,w} = \sum_{a \in V} {}^2D^3_{a,w} Y^1_{a,\gamma} Y^{3,*}_{a,\delta} \quad (3r_D r_T^2 N_v) \quad (12657)$$

$$\tau^8_{\gamma,a} = \sum_{b \in V} Y^3_{b,\gamma} \tau^7_{b,a} \quad (2r_T N_v^2) \quad (12670)$$

$$\tau^{12}_{\gamma,\delta,w,i} = \sum_{\epsilon \in A} \tau^{10}_{\epsilon,\gamma,i} \tau^{11}_{\epsilon,\delta,w} \quad (2r_D r_T^3 N_o) \quad (12658)$$

$$\tau^9_{\gamma,\delta,w} = \sum_{a \in V} {}^2D^1_{a,w} Y^{1,*}_{a,\delta} \tau^8_{\gamma,a} \quad (3r_D r_T^2 N_v) \quad (12671)$$

$$\tau^{13}_{\gamma,w,i} = \sum_{\delta \in A} \tau^2_{\delta,\gamma,w} \tau^{12}_{\delta,\gamma,w,i} \quad (2r_D r_T^2 N_o) \quad (12659)$$

$$\tau^{10}_{\gamma,\delta,w} = \sum_{i \in O} {}^2D^2_{i,w} Y^4_{i,\gamma} Y^{2,*}_{i,\delta} \quad (3r_D r_T^2 N_o) \quad (12672)$$

$${}^2R^4_{i,\gamma} \leftarrow - \sum_{w \in D} \frac{1}{2} {}^2D^4_{i,w} \tau^{13}_{\gamma,w,i} \quad (2r_D r_T N_o) \quad (12660)$$

Raw expression

$$\tau^{11}_{\gamma,\delta,w} = \sum_{\epsilon \in A} Z^*_{\epsilon,\delta} \tau^{10}_{\gamma,\epsilon,w} \tau^9_{\gamma,\epsilon,w} \quad (3r_D r_T^3) \quad (12673)$$

$${}^2R^4_{j,\zeta} \leftarrow - \sum_{\gamma \in A} \sum_{i \in O} \sum_{k \in O} \sum_{l \in O} \sum_{a \in V} \sum_{b \in V} \sum_{c \in V} \sum_{d \in V} \frac{1}{2} \quad (12661)$$

$$Y^{1,*}_{a,\gamma} Y^{2,*}_{i,\gamma} Z^*_{\gamma,\zeta} Y^{3,*}_{b,\zeta} {}^2D^{a,i,b,j}_{a,i,c,k} {}^2T_{a,i,c,k} {}^2T_{b,l,d,j} V_{k,c,l,d}$$

$$\tau^{12}_{\gamma,\delta,w} = \sum_{\epsilon \in A} Z_{\gamma,\epsilon} \tau^{11}_{\epsilon,\delta,w} \quad (2r_D r_T^3) \quad (12674)$$

Factorized expression

$${}^2R^4_{i,\gamma} \leftarrow - \sum_{\delta \in A} \sum_{w \in D} \frac{1}{2} {}^2D^4_{i,w} Y^2_{i,\delta} \tau^0_{\delta,\gamma,w} \tau^{12}_{\delta,\gamma,w} \quad (4r_D r_T^2 N_o) \quad (12675)$$

$$\tau^0_{\gamma,\delta,w} = \sum_{a \in V} {}^2D^3_{a,w} Y^1_{a,\gamma} Y^{3,*}_{a,\delta} \quad (3r_D r_T^2 N_v) \quad (12662)$$

Raw expression

$${}^2R^4_{j,\zeta} \leftarrow - \sum_{\gamma \in A} \sum_{i \in O} \sum_{k \in O} \sum_{l \in O} \sum_{a \in V} \sum_{b \in V} \sum_{c \in V} \sum_{d \in V} \frac{1}{2} \quad (12676)$$

$$Y^{1,*}_{a,\gamma} Y^{2,*}_{i,\gamma} Z^*_{\gamma,\zeta} Y^{3,*}_{b,\zeta}$$

$${}^2D^{a,i,b,j} {}^2T_{a,i,c,k} {}^2T_{d,j,b,l} V_{k,c,l,d}$$

Factorized expression

$$\tau^0_{\gamma,\delta,w} = \sum_{a \in V} {}^2D^1_{a,w} Y^1_{a,\gamma} Y^{1,*}_{a,\delta} \quad (3r_D r_T^2 N_v) \quad (12677)$$

$$\tau^1_{\gamma,\alpha} = \sum_{a \in V} W^4_{a,\alpha} Y^3_{a,\gamma} \quad (2r_T r_V N_v) \quad (12678)$$

$$\tau^2_{\gamma,\alpha} = \sum_{i \in O} W^3_{i,\alpha} Y^4_{i,\gamma} \quad (2r_T r_V N_o) \quad (12679)$$

$$\tau^3_{\gamma,\alpha} = \sum_{\beta \in B} X_{\alpha,\beta} \tau^1_{\gamma,\beta} \tau^2_{\gamma,\beta} \quad (3r_T r_V^2) \quad (12680)$$

$$\tau^4_{\gamma,\alpha} = \sum_{\delta \in A} Z_{\gamma,\delta} \tau^3_{\delta,\alpha} \quad (2r_T^2 r_V) \quad (12681)$$

$$\tau^5_{\gamma,\alpha} = \sum_{a \in V} W^2_{a,\alpha} Y^3_{a,\gamma} \quad (2r_T r_V N_v) \quad (12682)$$

$$\tau^6_{\gamma,\delta,i} = \sum_{\alpha \in B} W^1_{i,\alpha} \tau^4_{\gamma,\alpha} \tau^5_{\delta,\alpha} \quad (3r_T^2 r_V N_o) \quad (12683)$$

$$\tau^7_{\gamma,\delta,\epsilon} = \sum_{i \in O} Y^2_{i,\gamma} Z_{\gamma,\epsilon} \tau^6_{\delta,\epsilon,i} \quad (3r_T^3 N_o) \quad (12684)$$

$$\tau^8_{\gamma,\delta,i} = \sum_{\epsilon \in A} Y^4_{i,\epsilon} \tau^7_{\gamma,\delta,\epsilon} \quad (2r_T^3 N_o) \quad (12685)$$

$$\tau^9_{\gamma,\delta,w} = \sum_{\epsilon \in A} \sum_{i \in O} {}^2D^2_{i,w} Y^{2,*}_{i,\delta} \tau^0_{\epsilon,\delta,w} \tau^8_{\epsilon,\gamma,i} \quad (4r_D r_T^3 N_o) \quad (12686)$$

$$\tau^{10}_{\gamma,\delta,w} = \sum_{\epsilon \in A} Z^*_{\epsilon,\delta} \tau^9_{\gamma,\epsilon,w} \quad (2r_D r_T^3) \quad (12687)$$

$$\tau^{11}_{\gamma,\delta,w} = \sum_{a \in V} {}^2D^3_{a,w} Y^1_{a,\gamma} Y^{3,*}_{a,\delta} \quad (3r_D r_T^2 N_v) \quad (12688)$$

$${}^2R^4_{i,\gamma} \leftarrow - \sum_{\delta \in A} \sum_{w \in D} \frac{1}{2} {}^2D^4_{i,w} Y^2_{i,\delta} \tau^{10}_{\delta,\gamma,w} \tau^{11}_{\delta,\gamma,w} \quad (4r_D r_T^2 N_o) \quad (12689)$$

Raw expression

$${}^2R^4_{j,\zeta} \leftarrow - \sum_{\gamma \in A} \sum_{i \in O} \sum_{k \in O} \sum_{l \in O} \sum_{a \in V} \sum_{b \in V} \sum_{c \in V} \sum_{d \in V} \frac{1}{2} \quad (12690)$$

$$Y^{1,*}_{a,\gamma} Y^{2,*}_{i,\gamma} Z^*_{\gamma,\zeta} Y^{3,*}_{b,\zeta}$$

$${}^2D^{a,i,b,j} {}^2T_{a,i,c,k} {}^2T_{d,l,b,j} V_{k,d,l,c}$$

Factorized expression

$$\tau^0_{\gamma,\delta,w} = \sum_{a \in V} {}^2D^3_{a,w} Y^3_{a,\gamma} Y^{3,*}_{a,\delta} \quad (3r_D r_T^2 N_v) \quad (12691)$$

$$\tau^1_{\gamma,\delta,w} = \sum_{a \in V} {}^2D^1_{a,w} Y^1_{a,\gamma} Y^{1,*}_{a,\delta} \quad (3r_D r_T^2 N_v) \quad (12692)$$

$$\tau^2_{\gamma,\delta,w} = \sum_{i \in O} {}^2D^2_{i,w} Y^2_{i,\gamma} Y^{2,*}_{i,\delta} \quad (3r_D r_T^2 N_o) \quad (12693)$$

$$\tau^3_{\gamma,\delta,w} = \sum_{\epsilon \in A} Z^*_{\epsilon,\delta} \tau^1_{\gamma,\epsilon,w} \tau^2_{\gamma,\epsilon,w} \quad (3r_D r_T^3) \quad (12694)$$

$$\tau^4_{\gamma,\delta,w} = \sum_{\epsilon \in A} Z_{\epsilon,\gamma} \tau^3_{\epsilon,\delta,w} \quad (2r_D r_T^3) \quad (12695)$$

$$\tau^5_{\gamma,\alpha} = \sum_{a \in V} W^2_{a,\alpha} Y^1_{a,\gamma} \quad (2r_T r_V N_v) \quad (12696)$$

$$\tau^6_{\gamma,\alpha} = \sum_{a \in V} W^4_{a,\alpha} Y^3_{a,\gamma} \quad (2r_T r_V N_v) \quad (12697)$$

$$\tau^7_{\gamma,\alpha} = \sum_{i \in O} W^3_{i,\alpha} Y^4_{i,\gamma} \quad (2r_T r_V N_o) \quad (12698)$$

$$\tau^8_{\gamma,\alpha} = \sum_{\beta \in B} X_{\alpha,\beta} \tau^6_{\gamma,\beta} \tau^7_{\gamma,\beta} \quad (3r_T r_V^2) \quad (12699)$$

$$\tau^9_{\gamma,\alpha} = \sum_{\delta \in A} Z_{\gamma,\delta} \tau^8_{\delta,\alpha} \quad (2r_T^2 r_V) \quad (12700)$$

$$\tau^{10}_{\gamma,i} = \sum_{\alpha \in B} W^1_{i,\alpha} \tau^5_{\gamma,\alpha} \tau^9_{\gamma,\alpha} \quad (3r_T r_V N_o) \quad (12701)$$

$$\tau^{11}_{i,j} = \sum_{\gamma \in A} Y^2_{j,\gamma} \tau^{10}_{\gamma,i} \quad (2r_T N_o^2) \quad (12702)$$

$$\tau^9_{\gamma,a} = \sum_{\alpha \in B} W^4_{a,\alpha} \tau^7_{\gamma,\alpha} \tau^8_{\gamma,\alpha} \quad (3r_T r_V N_v) \quad (12715)$$

$$\tau^{12}_{\gamma,i} = \sum_{j \in O} Y^4_{j,\gamma} \tau^{11}_{j,i} \quad (2r_T N_o^2) \quad (12703)$$

$$\tau^{10}_{\gamma,\delta} = \sum_{a \in V} Y^3_{a,\delta} \tau^9_{\gamma,a} \quad (2r_T^2 N_v) \quad (12716)$$

$${}^2R^4_{i,\gamma} \leftarrow - \sum_{\delta \in A} \sum_{w \in D} \frac{1}{2} {}^2D^4_{i,w} \tau^{12}_{\delta,i} \tau^0_{\delta,\gamma,w} \tau^4_{\delta,\gamma,w} \quad (4r_D r_T^2 N_o) \quad (12704)$$

$$\tau^{11}_{\gamma,a} = \sum_{\delta \in A} Y^3_{a,\delta} \tau^{10}_{\delta,\gamma} \quad (2r_T^2 N_v) \quad (12717)$$

Raw expression

$$\tau^{12}_{\gamma,\delta,w} = \sum_{a \in V} {}^2D^3_{a,w} Y^{3,*}_{a,\delta} \tau^{11}_{\gamma,a} \quad (3r_D r_T^2 N_v) \quad (12718)$$

$${}^2R^4_{j,\zeta} \leftarrow - \sum_{\gamma \in A} \sum_{i \in O} \sum_{k \in O} \sum_{l \in O} \sum_{a \in V} \sum_{b \in V} \sum_{c \in V} \sum_{d \in V} \frac{1}{2} \quad (12705)$$

$$Y^{1,*}_{a,\gamma} \quad Y^{2,*}_{i,\gamma} \quad Z^*_{\gamma,\zeta} \quad Y^{3,*}_{b,\zeta}$$

$${}^2D^{a,i,b,j} \quad {}^2T_{a,i,d,j} \quad {}^2T_{b,k,c,l} \quad V_{k,d,l,c}$$

$${}^2R^4_{i,\gamma} \leftarrow - \sum_{\delta \in A} \sum_{w \in D} \frac{1}{2} {}^2D^4_{i,w} Y^4_{i,\delta} \tau^{12}_{\delta,\gamma,w} \tau^3_{\delta,\gamma,w} \quad (4r_D r_T^2 N_o) \quad (12719)$$

Factorized expression

Raw expression

$$\tau^0_{\gamma,\delta,w} = \sum_{a \in V} {}^2D^1_{a,w} Y^1_{a,\gamma} Y^{1,*}_{a,\delta} \quad (3r_D r_T^2 N_v) \quad (12706)$$

$${}^2R^4_{j,\zeta} \leftarrow - \sum_{\gamma \in A} \sum_{i \in O} \sum_{k \in O} \sum_{l \in O} \sum_{a \in V} \sum_{b \in V} \sum_{c \in V} \sum_{d \in V} \frac{1}{2} \quad (12720)$$

$$Y^{1,*}_{a,\gamma} \quad Y^{2,*}_{i,\gamma} \quad Z^*_{\gamma,\zeta} \quad Y^{3,*}_{b,\zeta}$$

$${}^2D^{a,i,b,j} \quad {}^2T_{a,i,d,j} \quad {}^2T_{c,k,b,l} \quad V_{k,c,l,d}$$

$$\tau^1_{\gamma,\delta,w} = \sum_{i \in O} {}^2D^2_{i,w} Y^2_{i,\gamma} Y^{2,*}_{i,\delta} \quad (3r_D r_T^2 N_o) \quad (12707)$$

Factorized expression

$$\tau^2_{\gamma,\delta,w} = \sum_{\epsilon \in A} Z^*_{\epsilon,\delta} \tau^0_{\gamma,\epsilon,w} \tau^1_{\gamma,\epsilon,w} \quad (3r_D r_T^3) \quad (12708)$$

$$\tau^0_{\gamma,\delta,w} = \sum_{a \in V} {}^2D^1_{a,w} Y^1_{a,\gamma} Y^{1,*}_{a,\delta} \quad (3r_D r_T^2 N_v) \quad (12721)$$

$$\tau^3_{\gamma,\delta,w} = \sum_{\epsilon \in A} Z_{\epsilon,\gamma} \tau^2_{\epsilon,\delta,w} \quad (2r_D r_T^3) \quad (12709)$$

$$\tau^1_{\gamma,\delta,w} = \sum_{i \in O} {}^2D^2_{i,w} Y^2_{i,\gamma} Y^{2,*}_{i,\delta} \quad (3r_D r_T^2 N_o) \quad (12722)$$

$$\tau^4_{\gamma,\alpha} = \sum_{a \in V} W^2_{a,\alpha} Y^1_{a,\gamma} \quad (2r_T r_V N_v) \quad (12710)$$

$$\tau^2_{\gamma,\delta,w} = \sum_{\epsilon \in A} Z^*_{\epsilon,\delta} \tau^0_{\gamma,\epsilon,w} \tau^1_{\gamma,\epsilon,w} \quad (3r_D r_T^3) \quad (12723)$$

$$\tau^5_{\gamma,\alpha} = \sum_{i \in O} W^1_{i,\alpha} Y^2_{i,\gamma} \quad (2r_T r_V N_o) \quad (12711)$$

$$\tau^3_{\gamma,\alpha} = \sum_{a \in V} W^2_{a,\alpha} Y^1_{a,\gamma} \quad (2r_T r_V N_v) \quad (12724)$$

$$\tau^6_{\gamma,\alpha} = \sum_{\beta \in B} X_{\beta,\alpha} \tau^4_{\gamma,\beta} \tau^5_{\gamma,\beta} \quad (3r_T r_V^2) \quad (12712)$$

$$\tau^4_{\gamma,\alpha,i} = \sum_{\beta \in B} W^1_{i,\beta} X_{\beta,\alpha} \tau^3_{\gamma,\beta} \quad (3r_T r_V^2 N_o) \quad (12725)$$

$$\tau^7_{\gamma,\alpha} = \sum_{\delta \in A} Z_{\delta,\gamma} \tau^6_{\delta,\alpha} \quad (2r_T^2 r_V) \quad (12713)$$

$$\tau^5_{\gamma,\alpha} = \sum_{i \in O} W^3_{i,\alpha} Y^2_{i,\gamma} \quad (2r_T r_V N_o) \quad (12726)$$

$$\tau^8_{\gamma,\alpha} = \sum_{i \in O} W^3_{i,\alpha} Y^4_{i,\gamma} \quad (2r_T r_V N_o) \quad (12714)$$

$$\tau^6_{\gamma,\alpha} = \sum_{a \in V} W^4_{a,\alpha} Y^3_{a,\gamma} \quad (2r_T r_V N_v) \quad (12727)$$

$$\tau_{\gamma,\delta,i}^7 = \sum_{\alpha \in B} \tau_{\gamma,\alpha}^5 \tau_{\delta,\alpha}^6 \tau_{\gamma,\alpha,i}^4 \quad (3r_T^2 r_V N_o) \quad (12728)$$

$$\tau_{\gamma,\alpha}^5 = \sum_{\delta \in A} Z_{\gamma,\delta} \tau_{\delta,\alpha}^4 \quad (2r_T^2 r_V) \quad (12741)$$

$$\tau_{\gamma,\delta}^8 = \sum_{i \in O} Y_{i,\delta}^4 \tau_{\gamma,\delta,i}^7 \quad (2r_T^2 N_o) \quad (12729)$$

$$\tau_{\gamma,i}^6 = \sum_{\alpha \in B} W_{i,\alpha}^1 \tau_{\gamma,\alpha}^1 \tau_{\gamma,\alpha}^5 \quad (3r_T r_V N_o) \quad (12742)$$

$$\tau_{\gamma,\delta}^9 = \sum_{\epsilon \in A} Z_{\delta,\epsilon} \tau_{\gamma,\epsilon}^8 \quad (2r_T^3) \quad (12730)$$

$$\tau_{i,j}^7 = \sum_{\gamma \in A} Y_{j,\gamma}^2 \tau_{\gamma,i}^6 \quad (2r_T N_o^2) \quad (12743)$$

$$\tau_{\gamma,\delta}^{10} = \sum_{\epsilon \in A} Z_{\epsilon,\delta} \tau_{\epsilon,\gamma}^9 \quad (2r_T^3) \quad (12731)$$

$$\tau_{\gamma,i}^8 = \sum_{j \in O} Y_{j,\gamma}^2 \tau_{j,i}^7 \quad (2r_T N_o^2) \quad (12744)$$

$$\tau_{\gamma,\delta,w}^{11} = \sum_{\epsilon \in A} \tau_{\epsilon,\gamma}^{10} \tau_{\epsilon,\delta,w}^2 \quad (2r_D r_T^3) \quad (12732)$$

$$\tau_{\gamma,\delta,w}^9 = \sum_{i \in O} {}^2D_{i,w}^2 Y_{i,\delta}^{2,*} \tau_{\gamma,i}^8 \quad (3r_D r_T^2 N_o) \quad (12745)$$

$$\tau_{\gamma,\delta,w}^{12} = \sum_{a \in V} {}^2D_{a,w}^3 Y_{a,\gamma}^3 Y_{a,\delta}^{3,*} \quad (3r_D r_T^2 N_v) \quad (12733)$$

$$\tau_{\gamma,\delta,w}^{10} = \sum_{a \in V} {}^2D_{a,w}^1 Y_{a,\gamma}^1 Y_{a,\delta}^{1,*} \quad (3r_D r_T^2 N_v) \quad (12746)$$

$${}^2R_{i,\gamma}^4 \leftarrow - \sum_{\delta \in A} \sum_{w \in D} \frac{1}{2} {}^2D_{i,w}^4 Y_{i,\delta}^4 \tau_{\delta,\gamma,w}^{11} \tau_{\delta,\gamma,w}^{12} \quad (4r_D r_T^2 N_o) \quad (12734)$$

$$\tau_{\gamma,\delta,w}^{12} = \sum_{\epsilon \in A} Z_{\epsilon,\gamma} \tau_{\epsilon,\delta,w}^{11} \quad (2r_D r_T^3) \quad (12748)$$

$${}^2R_{j,\zeta}^4 \leftarrow - \sum_{\gamma \in A} \sum_{i \in O} \sum_{k \in O} \sum_{l \in O} \sum_{a \in V} \sum_{b \in V} \sum_{c \in V} \sum_{d \in V} \frac{1}{2} \quad (12735)$$

$$Y_{a,\gamma}^{1,*} Y_{i,\gamma}^{2,*} Z_{\gamma,\zeta}^* Y_{b,\zeta}^{3,*} {}^2D_{a,i,b,j} {}^2T_{a,k,c,i} {}^2T_{b,j,d,l} V_{k,c,l,d}$$

$${}^2R_{i,\gamma}^4 \leftarrow - \sum_{\delta \in A} \sum_{w \in D} \frac{1}{2} {}^2D_{i,w}^4 Y_{i,\delta}^4 \tau_{\delta,\gamma,w}^0 \tau_{\delta,\gamma,w}^{12} \quad (4r_D r_T^2 N_o) \quad (12749)$$

Factorized expression

Raw expression

$$\tau_{\gamma,\delta,w}^0 = \sum_{a \in V} {}^2D_{a,w}^3 Y_{a,\gamma}^3 Y_{a,\delta}^{3,*} \quad (3r_D r_T^2 N_v) \quad (12736)$$

$${}^2R_{j,\zeta}^4 \leftarrow - \sum_{\gamma \in A} \sum_{i \in O} \sum_{k \in O} \sum_{l \in O} \sum_{a \in V} \sum_{b \in V} \sum_{c \in V} \sum_{d \in V} \frac{1}{2} \quad (12750)$$

$$Y_{a,\gamma}^{1,*} Y_{i,\gamma}^{2,*} Z_{\gamma,\zeta}^* Y_{b,\zeta}^{3,*} {}^2D_{a,i,b,j} {}^2T_{a,k,c,i} {}^2T_{d,l,b,j} V_{k,c,l,d}$$

$$\tau_{\gamma,\alpha}^1 = \sum_{a \in V} W_{a,\alpha}^2 Y_{a,\gamma}^1 \quad (2r_T r_V N_v) \quad (12737)$$

Factorized expression

$$\tau_{\gamma,\alpha}^2 = \sum_{a \in V} W_{a,\alpha}^4 Y_{a,\gamma}^3 \quad (2r_T r_V N_v) \quad (12738)$$

$$\tau_{\gamma,\delta,w}^0 = \sum_{a \in V} {}^2D_{a,w}^3 Y_{a,\gamma}^3 Y_{a,\delta}^{3,*} \quad (3r_D r_T^2 N_v) \quad (12751)$$

$$\tau_{\gamma,\alpha}^3 = \sum_{i \in O} W_{i,\alpha}^3 Y_{i,\gamma}^4 \quad (2r_T r_V N_o) \quad (12739)$$

$$\tau_{\gamma,\delta,w}^1 = \sum_{i \in O} {}^2D_{i,w}^2 Y_{i,\gamma}^2 Y_{i,\delta}^{2,*} \quad (3r_D r_T^2 N_o) \quad (12752)$$

$$\tau_{\gamma,\alpha}^4 = \sum_{\beta \in B} X_{\alpha,\beta} \tau_{\gamma,\beta}^2 \tau_{\gamma,\beta}^3 \quad (3r_T r_V^2) \quad (12740)$$

$$\tau_{\gamma,\alpha}^2 = \sum_{i \in O} W_{i,\alpha}^1 Y_{i,\gamma}^2 \quad (2r_T r_V N_o) \quad (12753)$$

$$\tau^3_{\gamma,\alpha} = \sum_{a \in V} W^4_{a,\alpha} Y^3_{a,\gamma} \quad (2r_T r_V N_v) \quad (12754)$$

$$\tau^1_{\gamma,\delta,w} = \sum_{i \in O} {}^2D^2_{i,w} Y^2_{i,\gamma} Y^{2,*}_{i,\delta} \quad (3r_D r_T^2 N_o) \quad (12767)$$

$$\tau^4_{\gamma,\alpha} = \sum_{i \in O} W^3_{i,\alpha} Y^4_{i,\gamma} \quad (2r_T r_V N_o) \quad (12755)$$

$$\tau^2_{\gamma,\delta,w} = \sum_{\epsilon \in A} Z^*_{\epsilon,\delta} \tau^0_{\gamma,\epsilon,w} \tau^1_{\gamma,\epsilon,w} \quad (3r_D r_T^3) \quad (12768)$$

$$\tau^5_{\gamma,\alpha} = \sum_{\beta \in B} X_{\alpha,\beta} \tau^3_{\gamma,\beta} \tau^4_{\gamma,\beta} \quad (3r_T r_V^2) \quad (12756)$$

$$\tau^3_{\gamma,\alpha} = \sum_{a \in V} W^4_{a,\alpha} Y^1_{a,\gamma} \quad (2r_T r_V N_v) \quad (12769)$$

$$\tau^6_{\gamma,\alpha} = \sum_{\delta \in A} Z_{\gamma,\delta} \tau^5_{\delta,\alpha} \quad (2r_T^2 r_V) \quad (12757)$$

$$\tau^4_{\gamma,\alpha} = \sum_{a \in V} W^2_{a,\alpha} Y^3_{a,\gamma} \quad (2r_T r_V N_v) \quad (12770)$$

$$\tau^7_{\gamma,a} = \sum_{\alpha \in B} W^2_{a,\alpha} \tau^2_{\gamma,\alpha} \tau^6_{\gamma,\alpha} \quad (3r_T r_V N_v) \quad (12758)$$

$$\tau^5_{\gamma,\alpha} = \sum_{i \in O} W^1_{i,\alpha} Y^4_{i,\gamma} \quad (2r_T r_V N_o) \quad (12771)$$

$$\tau^8_{a,b} = \sum_{\gamma \in A} Y^1_{b,\gamma} \tau^7_{\gamma,a} \quad (2r_T N_v^2) \quad (12759)$$

$$\tau^6_{\gamma,\alpha} = \sum_{\beta \in B} X_{\beta,\alpha} \tau^4_{\gamma,\beta} \tau^5_{\gamma,\beta} \quad (3r_T r_V^2) \quad (12772)$$

$$\tau^9_{\gamma,a} = \sum_{b \in V} Y^1_{b,\gamma} \tau^8_{b,a} \quad (2r_T N_v^2) \quad (12760)$$

$$\tau^7_{\gamma,\alpha} = \sum_{\delta \in A} Z_{\gamma,\delta} \tau^6_{\delta,\alpha} \quad (2r_T^2 r_V) \quad (12773)$$

$$\tau^{10}_{\gamma,\delta,w} = \sum_{a \in V} {}^2D^1_{a,w} Y^{1,*}_{a,\delta} \tau^9_{\gamma,a} \quad (3r_D r_T^2 N_v) \quad (12761)$$

$$\tau^8_{\gamma,\delta,i} = \sum_{\alpha \in B} W^3_{i,\alpha} \tau^3_{\gamma,\alpha} \tau^7_{\delta,\alpha} \quad (3r_T^2 r_V N_o) \quad (12774)$$

$$\tau^{11}_{\gamma,\delta,w} = \sum_{\epsilon \in A} Z^*_{\epsilon,\delta} \tau^1_{\gamma,\epsilon,w} \tau^{10}_{\gamma,\epsilon,w} \quad (3r_D r_T^3) \quad (12762)$$

$$\tau^9_{\gamma,\delta,\epsilon} = \sum_{i \in O} Z_{\gamma,\epsilon} Y^4_{i,\epsilon} \tau^8_{\gamma,\delta,i} \quad (3r_T^3 N_o) \quad (12775)$$

$$\tau^{12}_{\gamma,\delta,w} = \sum_{\epsilon \in A} Z_{\epsilon,\gamma} \tau^{11}_{\epsilon,\delta,w} \quad (2r_D r_T^3) \quad (12763)$$

$$\tau^{10}_{\gamma,\delta,i} = \sum_{\epsilon \in A} Y^2_{i,\epsilon} \tau^9_{\epsilon,\gamma,\delta} \quad (2r_T^3 N_o) \quad (12776)$$

$${}^2R^4_{i,\gamma} \leftarrow - \sum_{\delta \in A} \sum_{w \in D} \frac{1}{2} {}^2D^4_{i,w} Y^4_{i,\delta} \tau^0_{\delta,\gamma,w} \tau^{12}_{\delta,\gamma,w} \quad (4r_D r_T^2 N_o) \quad (12764)$$

$$\tau^{11}_{\gamma,\delta,w,i} = \sum_{\epsilon \in A} \tau^{10}_{\epsilon,\gamma,i} \tau^2_{\epsilon,\delta,w} \quad (2r_D r_T^3 N_o) \quad (12777)$$

Raw expression

$${}^2R^4_{j,\zeta} \leftarrow - \sum_{\gamma \in A} \sum_{i \in O} \sum_{k \in O} \sum_{l \in O} \sum_{a \in V} \sum_{b \in V} \sum_{c \in V} \sum_{d \in V} \frac{1}{2} \quad (12765)$$

$$Y^{1,*}_{a,\gamma} Y^{2,*}_{i,\gamma} Z^*_{\gamma,\zeta} Y^{3,*}_{b,\zeta} {}^2D^{a,i,b,j}_{a,k,c,l} {}^2T_{a,k,c,l} {}^2T_{b,j,d,i} V_{k,d,l,c}$$

$$\tau^{12}_{\gamma,\delta,w} = \sum_{a \in V} {}^2D^3_{a,w} Y^3_{a,\gamma} Y^{3,*}_{a,\delta} \quad (3r_D r_T^2 N_v) \quad (12778)$$

$$\tau^{13}_{\gamma,w,i} = \sum_{\delta \in A} \tau^{12}_{\delta,\gamma,w} \tau^{11}_{\delta,\gamma,w,i} \quad (2r_D r_T^2 N_o) \quad (12779)$$

Factorized expression

$$\tau^0_{\gamma,\delta,w} = \sum_{a \in V} {}^2D^1_{a,w} Y^1_{a,\gamma} Y^{1,*}_{a,\delta} \quad (3r_D r_T^2 N_v) \quad (12766)$$

$${}^2R^4_{i,\gamma} \leftarrow - \sum_{w \in D} \frac{1}{2} {}^2D^4_{i,w} \tau^{13}_{\gamma,w,i} \quad (2r_D r_T N_o) \quad (12780)$$

Raw expression



$${}^2R^4_{j,\zeta} \leftarrow - \sum_{\gamma \in A} \sum_{i \in O} \sum_{k \in O} \sum_{l \in O} \sum_{a \in V} \sum_{b \in V} \sum_{c \in V} \sum_{d \in V} \frac{1}{2} \quad (12781)$$

$$Y^{1,*}_{a,\gamma} \ Y^{2,*}_{i,\gamma} \ Z^*_{\gamma,\zeta} \ Y^{3,*}_{b,\zeta}$$

$${}^2D^{a,i,b,j} \ {}^2T_{a,k,c,l} \ {}^2T_{d,i,b,j} \ V_{k,d,l,c}$$

Factorized expression

$$\tau^0_{\gamma,\delta,w} = \sum_{a \in V} {}^2D^3_{a,w} Y^3_{a,\gamma} Y^{3,*}_{a,\delta} \quad (3r_D r_T^2 N_v) \quad (12782)$$

$$\tau^1_{\gamma,\delta,w} = \sum_{a \in V} {}^2D^1_{a,w} Y^1_{a,\gamma} Y^{1,*}_{a,\delta} \quad (3r_D r_T^2 N_v) \quad (12783)$$

$$\tau^2_{\gamma,\delta,w} = \sum_{i \in O} {}^2D^2_{i,w} Y^2_{i,\gamma} Y^{2,*}_{i,\delta} \quad (3r_D r_T^2 N_o) \quad (12784)$$

$$\tau^3_{\gamma,\delta,w} = \sum_{\epsilon \in A} Z^*_{\epsilon,\delta} \tau^1_{\gamma,\epsilon,w} \tau^2_{\gamma,\epsilon,w} \quad (3r_D r_T^3) \quad (12785)$$

$$\tau^4_{\gamma,\delta,w} = \sum_{\epsilon \in A} Z_{\epsilon,\gamma} \tau^3_{\epsilon,\delta,w} \quad (2r_D r_T^3) \quad (12786)$$

$$\tau^5_{\gamma,\alpha} = \sum_{a \in V} W^4_{a,\alpha} Y^1_{a,\gamma} \quad (2r_T r_V N_v) \quad (12787)$$

$$\tau^6_{\gamma,\alpha} = \sum_{i \in O} W^3_{i,\alpha} Y^2_{i,\gamma} \quad (2r_T r_V N_o) \quad (12788)$$

$$\tau^7_{\gamma,\alpha} = \sum_{\beta \in B} X_{\alpha,\beta} \tau^5_{\gamma,\beta} \tau^6_{\gamma,\beta} \quad (3r_T r_V^2) \quad (12789)$$

$$\tau^8_{\gamma,\alpha} = \sum_{\delta \in A} Z_{\delta,\gamma} \tau^7_{\delta,\alpha} \quad (2r_T^2 r_V) \quad (12790)$$

$$\tau^9_{\gamma,\alpha} = \sum_{a \in V} W^2_{a,\alpha} Y^3_{a,\gamma} \quad (2r_T r_V N_v) \quad (12791)$$

$$\tau^{10}_{\gamma,i} = \sum_{\alpha \in B} W^1_{i,\alpha} \tau^8_{\gamma,\alpha} \tau^9_{\gamma,\alpha} \quad (3r_T r_V N_o) \quad (12792)$$

$$\tau^{11}_{i,j} = \sum_{\gamma \in A} Y^4_{j,\gamma} \tau^{10}_{\gamma,i} \quad (2r_T N_o^2) \quad (12793)$$

$$\tau^{12}_{\gamma,i} = \sum_{j \in O} Y^4_{j,\gamma} \tau^{11}_{j,i} \quad (2r_T N_o^2) \quad (12794)$$

$${}^2R^4_{i,\gamma} \leftarrow - \sum_{\delta \in A} \sum_{w \in D} \frac{1}{2} {}^2D^4_{i,w} \tau^{12}_{\delta,i} \tau^0_{\delta,\gamma,w} \tau^4_{\delta,\gamma,w} \quad (4r_D r_T^2 N_o) \quad (12795)$$

Raw expression

$${}^2R^4_{j,\zeta} \leftarrow - \sum_{\gamma \in A} \sum_{i \in O} \sum_{k \in O} \sum_{l \in O} \sum_{a \in V} \sum_{b \in V} \sum_{c \in V} \sum_{d \in V} \frac{1}{2} \quad (12796)$$

$$Y^{1,*}_{a,\gamma} \ Y^{2,*}_{i,\gamma} \ Z^*_{\gamma,\zeta} \ Y^{3,*}_{b,\zeta}$$

$${}^2D^{a,i,b,j} \ {}^2T_{a,l,b,j} \ {}^2T_{c,i,d,k} \ V_{l,c,k,d}$$

Factorized expression

$$\tau^0_{\gamma,\delta,w} = \sum_{a \in V} {}^2D^1_{a,w} Y^1_{a,\gamma} Y^{1,*}_{a,\delta} \quad (3r_D r_T^2 N_v) \quad (12797)$$

$$\tau^1_{\gamma,\alpha} = \sum_{a \in V} W^2_{a,\alpha} Y^3_{a,\gamma} \quad (2r_T r_V N_v) \quad (12798)$$

$$\tau^2_{\gamma,\alpha} = \sum_{a \in V} W^4_{a,\alpha} Y^1_{a,\gamma} \quad (2r_T r_V N_v) \quad (12799)$$

$$\tau^3_{\gamma,\alpha} = \sum_{i \in O} W^3_{i,\alpha} Y^2_{i,\gamma} \quad (2r_T r_V N_o) \quad (12800)$$

$$\tau^4_{\gamma,\alpha} = \sum_{\beta \in B} X_{\alpha,\beta} \tau^2_{\gamma,\beta} \tau^3_{\gamma,\beta} \quad (3r_T r_V^2) \quad (12801)$$

$$\tau^5_{\gamma,\alpha} = \sum_{\delta \in A} Z_{\delta,\gamma} \tau^4_{\delta,\alpha} \quad (2r_T^2 r_V) \quad (12802)$$

$$\tau^6_{\gamma,\delta,i} = \sum_{\alpha \in B} W^1_{i,\alpha} \tau^1_{\delta,\alpha} \tau^5_{\gamma,\alpha} \quad (3r_T^2 r_V N_o) \quad (12803)$$

$$\tau^7_{\gamma,\delta,\epsilon} = \sum_{i \in O} Y^2_{i,\gamma} \tau^6_{\delta,\epsilon,i} \quad (2r_T^3 N_o) \quad (12804)$$

$$\tau^8_{\gamma,\delta,i} = \sum_{\epsilon \in A} Z_{\gamma,\epsilon} Y^4_{i,\epsilon} \tau^7_{\gamma,\delta,\epsilon} \quad (3r_T^3 N_o) \quad (12805)$$

$$\tau^9_{\gamma,\delta,w} = \sum_{\epsilon \in A} \sum_{i \in O} {}^2D^2_{i,w} Y^{2,*}_{i,\delta} \tau^0_{\epsilon,\delta,w} \tau^8_{\epsilon,\gamma,i} \quad (4r_D r_T^3 N_o) \quad (12806)$$

$$\tau_{\gamma,\delta,w}^{10} = \sum_{\epsilon \in A} Z_{\epsilon,\delta}^* \tau_{\gamma,\epsilon,w}^9 \quad (2r_D r_T^3) \quad (12807)$$

$$\tau_{\gamma,i}^8 = \sum_{j \in O} Y_{j,\gamma}^2 \tau_{j,i}^7 \quad (2r_T N_o^2) \quad (12819)$$

$$\tau_{\gamma,\delta,w}^{11} = \sum_{a \in V} {}^2D_{a,w}^3 Y_{a,\gamma}^3 Y_{a,\delta}^{3,*} \quad (3r_D r_T^2 N_v) \quad (12808)$$

$$\tau_{\gamma,\delta,w}^9 = \sum_{i \in O} {}^2D_{i,w}^2 Y_{i,\delta}^{2,*} \tau_{\gamma,i}^8 \quad (3r_D r_T^2 N_o) \quad (12820)$$

$${}^2R_{i,\gamma}^4 \leftarrow - \sum_{\delta \in A} \sum_{w \in D} \frac{1}{2} {}^2D_{i,w}^4 Y_{i,\delta}^4 \tau_{\delta,\gamma,w}^{10} \tau_{\delta,\gamma,w}^{11} \quad (4r_D r_T^2 N_o) \quad (12809)$$

$$\tau_{\gamma,\delta,w}^{10} = \sum_{a \in V} {}^2D_{a,w}^1 Y_{a,\gamma}^1 Y_{a,\delta}^{1,*} \quad (3r_D r_T^2 N_v) \quad (12821)$$

Raw expression

$$\tau_{\gamma,\delta,w}^{11} = \sum_{\epsilon \in A} Z_{\epsilon,\delta}^* \tau_{\gamma,\epsilon,w}^{10} \tau_{\gamma,\epsilon,w}^9 \quad (3r_D r_T^3) \quad (12822)$$

$${}^2R_{j,\zeta}^4 \leftarrow - \sum_{\gamma \in A} \sum_{i \in O} \sum_{k \in O} \sum_{l \in O} \sum_{a \in V} \sum_{b \in V} \sum_{c \in V} \sum_{d \in V} \frac{1}{2} \quad (12810)$$

$$Y_{a,\gamma}^{1,*} Y_{i,\gamma}^{2,*} Z_{\gamma,\zeta}^* Y_{b,\zeta}^{3,*}$$

$${}^2D_{a,i,b,j} {}^2T_{a,l,b,j} {}^2T_{c,k,d,i} V_{l,d,k,c}$$

$$\tau_{\gamma,\delta,w}^{12} = \sum_{\epsilon \in A} Z_{\epsilon,\gamma} \tau_{\epsilon,\delta,w}^{11} \quad (2r_D r_T^3) \quad (12823)$$

$${}^2R_{i,\gamma}^4 \leftarrow - \sum_{\delta \in A} \sum_{w \in D} \frac{1}{2} {}^2D_{i,w}^4 Y_{i,\delta}^4 \tau_{\delta,\gamma,w}^0 \tau_{\delta,\gamma,w}^{12} \quad (4r_D r_T^2 N_o) \quad (12824)$$

Factorized expression

$$\tau_{\gamma,\delta,w}^0 = \sum_{a \in V} {}^2D_{a,w}^3 Y_{a,\gamma}^3 Y_{a,\delta}^{3,*} \quad (3r_D r_T^2 N_v) \quad (12811)$$

Raw expression

$${}^2R_{j,\zeta}^4 \leftarrow - \sum_{\gamma \in A} \sum_{i \in O} \sum_{k \in O} \sum_{l \in O} \sum_{a \in V} \sum_{b \in V} \sum_{c \in V} \sum_{d \in V} \frac{1}{2} \quad (12825)$$

$$Y_{a,\gamma}^{1,*} Y_{i,\gamma}^{2,*} Z_{\gamma,\zeta}^* Y_{b,\zeta}^{3,*}$$

$${}^2D_{a,i,b,j} {}^2T_{b,j,a,l} {}^2T_{c,i,d,k} V_{l,c,k,d}$$

Factorized expression

$$\tau_{\gamma,\alpha}^2 = \sum_{i \in O} W_{i,\alpha}^3 Y_{i,\gamma}^2 \quad (2r_T r_V N_o) \quad (12813)$$

$$\tau_{\gamma,\alpha}^0 = \sum_{i \in O} W_{i,\alpha}^1 Y_{i,\gamma}^2 \quad (2r_T r_V N_o) \quad (12826)$$

$$\tau_{\gamma,\alpha}^3 = \sum_{\beta \in B} X_{\alpha,\beta} \tau_{\gamma,\beta}^1 \tau_{\gamma,\beta}^2 \quad (3r_T r_V^2) \quad (12814)$$

$$\tau_{\gamma,\alpha}^1 = \sum_{a \in V} W_{a,\alpha}^4 Y_{a,\gamma}^3 \quad (2r_T r_V N_v) \quad (12827)$$

$$\tau_{\gamma,\alpha}^4 = \sum_{\delta \in A} Z_{\delta,\gamma} \tau_{\delta,\alpha}^3 \quad (2r_T^2 r_V) \quad (12815)$$

$$\tau_{\gamma,\alpha}^2 = \sum_{i \in O} W_{i,\alpha}^3 Y_{i,\gamma}^4 \quad (2r_T r_V N_o) \quad (12828)$$

$$\tau_{\gamma,\alpha}^5 = \sum_{a \in V} W_{a,\alpha}^2 Y_{a,\gamma}^3 \quad (2r_T r_V N_v) \quad (12816)$$

$$\tau_{\gamma,\alpha}^3 = \sum_{\beta \in B} X_{\alpha,\beta} \tau_{\gamma,\beta}^1 \tau_{\gamma,\beta}^2 \quad (3r_T r_V^2) \quad (12829)$$

$$\tau_{\gamma,i}^6 = \sum_{\alpha \in B} W_{i,\alpha}^1 \tau_{\gamma,\alpha}^4 \tau_{\gamma,\alpha}^5 \quad (3r_T r_V N_o) \quad (12817)$$

$$\tau_{\gamma,\alpha}^4 = \sum_{\delta \in A} Z_{\gamma,\delta} \tau_{\delta,\alpha}^3 \quad (2r_T^2 r_V) \quad (12830)$$

$$\tau_{i,j}^7 = \sum_{\gamma \in A} Y_{j,\gamma}^4 \tau_{\gamma,i}^6 \quad (2r_T N_o^2) \quad (12818)$$

$$\tau_{\gamma,a}^5 = \sum_{\alpha \in B} W_{a,\alpha}^2 \tau_{\gamma,\alpha}^0 \tau_{\gamma,\alpha}^4 \quad (3r_T r_V N_v) \quad (12831)$$

$$\tau_{a,b}^6 = \sum_{\gamma \in A} Y_{b,\gamma}^1 \tau_{\gamma,a}^5 \quad (2r_T N_v^2) \quad (12832)$$

$$\tau_{\gamma,a}^7 = \sum_{b \in V} Y_{b,\gamma}^1 \tau_{b,a}^6 \quad (2r_T N_v^2) \quad (12833)$$

$$\tau_{\gamma,\delta,w}^8 = \sum_{a \in V} {}^2D_{a,w}^3 Y_{a,\delta}^{3,*} \tau_{\gamma,a}^7 \quad (3r_D r_T^2 N_v) \quad (12834)$$

$$\tau_{\gamma,\delta,w}^9 = \sum_{a \in V} {}^2D_{a,w}^1 Y_{a,\gamma}^3 Y_{a,\delta}^{1,*} \quad (3r_D r_T^2 N_v) \quad (12835)$$

$$\tau_{\gamma,\delta,w}^{10} = \sum_{i \in O} {}^2D_{i,w}^2 Y_{i,\gamma}^4 Y_{i,\delta}^{2,*} \quad (3r_D r_T^2 N_o) \quad (12836)$$

$$\tau_{\gamma,\delta,w}^{11} = \sum_{\epsilon \in A} Z_{\epsilon,\delta}^* \tau_{\gamma,\epsilon,w}^{10} \tau_{\gamma,\epsilon,w}^9 \quad (3r_D r_T^3) \quad (12837)$$

$$\tau_{\gamma,\delta,w}^{12} = \sum_{\epsilon \in A} Z_{\gamma,\epsilon} \tau_{\epsilon,\delta,w}^{11} \quad (2r_D r_T^3) \quad (12838)$$

$${}^2R_{i,\gamma}^4 \leftarrow - \sum_{\delta \in A} \sum_{w \in D} \frac{1}{2} {}^2D_{i,w}^4 Y_{i,\delta}^2 \tau_{\delta,\gamma,w}^{12} \tau_{\delta,\gamma,w}^8 \quad (4r_D r_T^2 N_o) \quad (12839)$$

Raw expression

$${}^2R_{j,\zeta}^4 \leftarrow - \sum_{\gamma \in A} \sum_{i \in O} \sum_{k \in O} \sum_{l \in O} \sum_{a \in V} \sum_{b \in V} \sum_{c \in V} \sum_{d \in V} \frac{1}{2} Y_{a,\gamma}^{1,*} Y_{i,\gamma}^{2,*} Z_{\gamma,\zeta}^* Y_{b,\zeta}^{3,*} {}^2D_{a,i,b,j}^{a,i,b,j} {}^2T_{b,j,a,l} {}^2T_{c,k,d,i} V_{l,d,k,c} \quad (12840)$$

Factorized expression

$$\tau_{\gamma,\delta,w}^0 = \sum_{a \in V} {}^2D_{a,w}^3 Y_{a,\gamma}^1 Y_{a,\delta}^{3,*} \quad (3r_D r_T^2 N_v) \quad (12841)$$

$$\tau_{\gamma,\delta,w}^1 = \sum_{a \in V} {}^2D_{a,w}^1 Y_{a,\gamma}^3 Y_{a,\delta}^{1,*} \quad (3r_D r_T^2 N_v) \quad (12842)$$

$$\tau_{\gamma,\delta,w}^2 = \sum_{i \in O} {}^2D_{i,w}^2 Y_{i,\gamma}^4 Y_{i,\delta}^{2,*} \quad (3r_D r_T^2 N_o) \quad (12843)$$

$$\tau_{\gamma,\delta,w}^3 = \sum_{\epsilon \in A} Z_{\epsilon,\delta}^* \tau_{\gamma,\epsilon,w}^1 \tau_{\gamma,\epsilon,w}^2 \quad (3r_D r_T^3) \quad (12844)$$

$$\tau_{\gamma,\delta,w}^4 = \sum_{\epsilon \in A} Z_{\gamma,\epsilon} \tau_{\epsilon,\delta,w}^3 \quad (2r_D r_T^3) \quad (12845)$$

$$\tau_{\gamma,\alpha}^5 = \sum_{a \in V} W_{a,\alpha}^2 Y_{a,\gamma}^1 \quad (2r_T r_V N_v) \quad (12846)$$

$$\tau_{\gamma,\alpha}^6 = \sum_{a \in V} W_{a,\alpha}^4 Y_{a,\gamma}^3 \quad (2r_T r_V N_v) \quad (12847)$$

$$\tau_{\gamma,\alpha}^7 = \sum_{i \in O} W_{i,\alpha}^3 Y_{i,\gamma}^4 \quad (2r_T r_V N_o) \quad (12848)$$

$$\tau_{\gamma,\alpha}^8 = \sum_{\beta \in B} X_{\alpha,\beta} \tau_{\gamma,\beta}^6 \tau_{\gamma,\beta}^7 \quad (3r_T r_V^2) \quad (12849)$$

$$\tau_{\gamma,\alpha}^9 = \sum_{\delta \in A} Z_{\gamma,\delta} \tau_{\delta,\alpha}^8 \quad (2r_T^2 r_V) \quad (12850)$$

$$\tau_{\gamma,i}^{10} = \sum_{\alpha \in B} W_{i,\alpha}^1 \tau_{\gamma,\alpha}^5 \tau_{\gamma,\alpha}^9 \quad (3r_T r_V N_o) \quad (12851)$$

$$\tau_{i,j}^{11} = \sum_{\gamma \in A} Y_{j,\gamma}^2 \tau_{\gamma,i}^{10} \quad (2r_T N_o^2) \quad (12852)$$

$$\tau_{\gamma,i}^{12} = \sum_{j \in O} Y_{j,\gamma}^2 \tau_{j,i}^{11} \quad (2r_T N_o^2) \quad (12853)$$

$${}^2R_{i,\gamma}^4 \leftarrow - \sum_{\delta \in A} \sum_{w \in D} \frac{1}{2} {}^2D_{i,w}^4 \tau_{\delta,i}^{12} \tau_{\delta,\gamma,w}^0 \tau_{\delta,\gamma,w}^4 \quad (4r_D r_T^2 N_o) \quad (12854)$$

Raw expression

$${}^2R_{j,\zeta}^4 \leftarrow - \sum_{\gamma \in A} \sum_{i \in O} \sum_{k \in O} \sum_{l \in O} \sum_{a \in V} \sum_{b \in V} \sum_{c \in V} \sum_{d \in V} \frac{1}{2} Y_{a,\gamma}^{1,*} Y_{i,\gamma}^{2,*} Z_{\gamma,\zeta}^* Y_{b,\zeta}^{3,*} {}^2D_{a,i,b,j}^{a,i,b,j} {}^2T_{b,j,d,i} {}^2T_{c,k,a,l} V_{k,c,l,d} \quad (12855)$$

Factorized expression

$$\tau_{\gamma,\delta,w}^0 = \sum_{a \in V} {}^2D_{a,w}^3 Y_{a,\gamma}^1 Y_{a,\delta}^{3,*} \quad (3r_D r_T^2 N_v) \quad (12856)$$

Factorized expression

$$\tau^1_{\gamma,\delta,w} = \sum_{a \in V} {}^2D^1_{a,w} Y^3_{a,\gamma} Y^{1,*}_{a,\delta} \quad (3r_D r_T^2 N_v) \quad (12857)$$

$$\tau^2_{\gamma,\delta,w} = \sum_{i \in O} {}^2D^2_{i,w} Y^4_{i,\gamma} Y^{2,*}_{i,\delta} \quad (3r_D r_T^2 N_o) \quad (12858)$$

$$\tau^3_{\gamma,\delta,w} = \sum_{\epsilon \in A} Z^*_{\epsilon,\delta} \tau^1_{\gamma,\epsilon,w} \tau^2_{\gamma,\epsilon,w} \quad (3r_D r_T^3) \quad (12859)$$

$$\tau^4_{\gamma,\delta,w} = \sum_{\epsilon \in A} Z_{\gamma,\epsilon} \tau^3_{\epsilon,\delta,w} \quad (2r_D r_T^3) \quad (12860)$$

$$\tau^5_{\gamma,\alpha} = \sum_{a \in V} W^4_{a,\alpha} Y^1_{a,\gamma} \quad (2r_T r_V N_v) \quad (12861)$$

$$\tau^6_{\gamma,\alpha} = \sum_{i \in O} W^3_{i,\alpha} Y^2_{i,\gamma} \quad (2r_T r_V N_o) \quad (12862)$$

$$\tau^7_{\gamma,\alpha} = \sum_{\beta \in B} X_{\alpha,\beta} \tau^5_{\gamma,\beta} \tau^6_{\gamma,\beta} \quad (3r_T r_V^2) \quad (12863)$$

$$\tau^8_{\gamma,\alpha} = \sum_{\delta \in A} Z_{\delta,\gamma} \tau^7_{\delta,\alpha} \quad (2r_T^2 r_V) \quad (12864)$$

$$\tau^9_{\gamma,\alpha} = \sum_{a \in V} W^2_{a,\alpha} Y^3_{a,\gamma} \quad (2r_T r_V N_v) \quad (12865)$$

$$\tau^{10}_{\gamma,i} = \sum_{\alpha \in B} W^1_{i,\alpha} \tau^8_{\gamma,\alpha} \tau^9_{\gamma,\alpha} \quad (3r_T r_V N_o) \quad (12866)$$

$$\tau^{11}_{i,j} = \sum_{\gamma \in A} Y^4_{j,\gamma} \tau^{10}_{\gamma,i} \quad (2r_T N_o^2) \quad (12867)$$

$$\tau^{12}_{\gamma,i} = \sum_{j \in O} Y^2_{j,\gamma} \tau^{11}_{j,i} \quad (2r_T N_o^2) \quad (12868)$$

$${}^2R^4_{i,\gamma} \leftarrow - \sum_{\delta \in A} \sum_{w \in D} \frac{1}{2} {}^2D^4_{i,w} \tau^{12}_{\delta,i} \tau^0_{\delta,\gamma,w} \tau^4_{\delta,\gamma,w} \quad (4r_D r_T^2 N_o) \quad (12869)$$

Raw expression

$${}^2R^4_{j,\zeta} \leftarrow - \sum_{\gamma \in A} \sum_{i \in O} \sum_{k \in O} \sum_{l \in O} \sum_{a \in V} \sum_{b \in V} \sum_{c \in V} \sum_{d \in V} \frac{1}{2} \quad (12870)$$

$$Y^{1,*}_{a,\gamma} Y^{2,*}_{i,\gamma} Z^*_{\gamma,\zeta} Y^{3,*}_{b,\zeta} {}^2D^{a,i,b,j} {}^2T_{b,j,d,l} {}^2T_{c,i,a,k} V_{k,c,l,d}$$

$$\tau^0_{\gamma,\delta,w} = \sum_{a \in V} {}^2D^3_{a,w} Y^1_{a,\gamma} Y^{3,*}_{a,\delta} \quad (3r_D r_T^2 N_v) \quad (12871)$$

$$\tau^1_{\gamma,\delta,w} = \sum_{a \in V} {}^2D^1_{a,w} Y^3_{a,\gamma} Y^{1,*}_{a,\delta} \quad (3r_D r_T^2 N_v) \quad (12872)$$

$$\tau^2_{\gamma,\alpha} = \sum_{a \in V} W^2_{a,\alpha} Y^1_{a,\gamma} \quad (2r_T r_V N_v) \quad (12873)$$

$$\tau^3_{\gamma,\alpha} = \sum_{a \in V} W^4_{a,\alpha} Y^3_{a,\gamma} \quad (2r_T r_V N_v) \quad (12874)$$

$$\tau^4_{\gamma,\alpha} = \sum_{i \in O} W^3_{i,\alpha} Y^4_{i,\gamma} \quad (2r_T r_V N_o) \quad (12875)$$

$$\tau^5_{\gamma,\alpha} = \sum_{\beta \in B} X_{\alpha,\beta} \tau^3_{\gamma,\beta} \tau^4_{\gamma,\beta} \quad (3r_T r_V^2) \quad (12876)$$

$$\tau^6_{\gamma,\alpha} = \sum_{\delta \in A} Z_{\gamma,\delta} \tau^5_{\delta,\alpha} \quad (2r_T^2 r_V) \quad (12877)$$

$$\tau^7_{\gamma,i} = \sum_{\alpha \in B} W^1_{i,\alpha} \tau^2_{\gamma,\alpha} \tau^6_{\gamma,\alpha} \quad (3r_T r_V N_o) \quad (12878)$$

$$\tau^8_{i,j} = \sum_{\gamma \in A} Y^2_{j,\gamma} \tau^7_{\gamma,i} \quad (2r_T N_o^2) \quad (12879)$$

$$\tau^9_{\gamma,i} = \sum_{j \in O} Y^4_{j,\gamma} \tau^8_{j,i} \quad (2r_T N_o^2) \quad (12880)$$

$$\tau^{10}_{\gamma,\delta,w} = \sum_{i \in O} {}^2D^2_{i,w} Y^{2,*}_{i,\delta} \tau^9_{\gamma,i} \quad (3r_D r_T^2 N_o) \quad (12881)$$

$$\tau^{11}_{\gamma,\delta,w} = \sum_{\epsilon \in A} Z^*_{\epsilon,\delta} \tau^1_{\gamma,\epsilon,w} \tau^{10}_{\gamma,\epsilon,w} \quad (3r_D r_T^3) \quad (12882)$$

$$\tau^{12}_{\gamma,\delta,w} = \sum_{\epsilon \in A} Z_{\gamma,\epsilon} \tau^{11}_{\epsilon,\delta,w} \quad (2r_D r_T^3) \quad (12883)$$

$${}^2R^4_{i,\gamma} \leftarrow - \sum_{\delta \in A} \sum_{w \in D} \frac{1}{2} {}^2D^4_{i,w} Y^2_{i,\delta} \tau^0_{\delta,\gamma,w} \tau^{12}_{\delta,\gamma,w} \quad (4r_D r_T^2 N_o) \quad (12884)$$

Raw expression

$${}^2R^4_{j,\zeta} \leftarrow - \sum_{\gamma \in A} \sum_{i \in O} \sum_{k \in O} \sum_{l \in O} \sum_{a \in V} \sum_{b \in V} \sum_{c \in V} \sum_{d \in V} \frac{1}{2} \quad (12885)$$

$$Y^{1,*}_{a,\gamma} \ Y^{2,*}_{i,\gamma} \ Z^*_{\gamma,\zeta} \ Y^{3,*}_{b,\zeta}$$

$${}^2D^{a,i,b,j} \ {}^2T_{b,j,d,l} \ {}^2T_{c,k,a,i} \ V_{k,d,l,c}$$

Factorized expression

$$\tau^0_{\gamma,\delta,w} = \sum_{a \in V} {}^2D^1_{a,w} Y^3_{a,\gamma} Y^{1,*}_{a,\delta} \quad (3r_D r_T^2 N_v) \quad (12886)$$

$$\tau^1_{\gamma,\alpha} = \sum_{a \in V} W^4_{a,\alpha} Y^3_{a,\gamma} \quad (2r_T r_V N_v) \quad (12887)$$

$$\tau^2_{\gamma,\alpha} = \sum_{i \in O} W^3_{i,\alpha} Y^4_{i,\gamma} \quad (2r_T r_V N_o) \quad (12888)$$

$$\tau^3_{\gamma,\alpha} = \sum_{\beta \in B} X_{\alpha,\beta} \tau^1_{\gamma,\beta} \tau^2_{\gamma,\beta} \quad (3r_T r_V^2) \quad (12889)$$

$$\tau^4_{\gamma,\alpha} = \sum_{\delta \in A} Z_{\gamma,\delta} \tau^3_{\delta,\alpha} \quad (2r_T^2 r_V) \quad (12890)$$

$$\tau^5_{\gamma,\alpha} = \sum_{a \in V} W^2_{a,\alpha} Y^1_{a,\gamma} \quad (2r_T r_V N_v) \quad (12891)$$

$$\tau^6_{\gamma,\delta,i} = \sum_{\alpha \in B} W^1_{i,\alpha} \tau^4_{\delta,\alpha} \tau^5_{\gamma,\alpha} \quad (3r_T^2 r_V N_o) \quad (12892)$$

$$\tau^7_{\gamma,\delta,\epsilon} = \sum_{i \in O} Z_{\gamma,\epsilon} Y^4_{i,\epsilon} \tau^6_{\gamma,\delta,i} \quad (3r_T^3 N_o) \quad (12893)$$

$$\tau^8_{\gamma,\delta,i} = \sum_{\epsilon \in A} Y^2_{i,\epsilon} \tau^7_{\epsilon,\gamma,\delta} \quad (2r_T^3 N_o) \quad (12894)$$

$$\tau^9_{\gamma,\delta,w} = \sum_{\epsilon \in A} \sum_{i \in O} {}^2D^2_{i,w} Y^{2,*}_{i,\delta} \tau^0_{\epsilon,\delta,w} \tau^8_{\gamma,\epsilon,i} \quad (4r_D r_T^3 N_o) \quad (12895)$$

$$\tau^{10}_{\gamma,\delta,w} = \sum_{\epsilon \in A} Z^*_{\epsilon,\delta} \tau^9_{\gamma,\epsilon,w} \quad (2r_D r_T^3) \quad (12896)$$

$$\tau^{11}_{\gamma,\delta,w} = \sum_{a \in V} {}^2D^3_{a,w} Y^1_{a,\gamma} Y^{3,*}_{a,\delta} \quad (3r_D r_T^2 N_v) \quad (12897)$$

$${}^2R^4_{i,\gamma} \leftarrow - \sum_{\delta \in A} \sum_{w \in D} \frac{1}{2} {}^2D^4_{i,w} Y^2_{i,\delta} \tau^{10}_{\delta,\gamma,w} \tau^{11}_{\delta,\gamma,w} \quad (4r_D r_T^2 N_o) \quad (12898)$$

Raw expression

$${}^2R^4_{j,\zeta} \leftarrow - \sum_{\gamma \in A} \sum_{i \in O} \sum_{k \in O} \sum_{l \in O} \sum_{a \in V} \sum_{b \in V} \sum_{c \in V} \sum_{d \in V} \frac{1}{2} \quad (12899)$$

$$Y^{1,*}_{a,\gamma} \ Y^{2,*}_{i,\gamma} \ Z^*_{\gamma,\zeta} \ Y^{3,*}_{b,\zeta}$$

$${}^2D^{a,i,b,j} \ {}^2T_{b,k,a,i} \ {}^2T_{c,j,d,l} \ V_{k,c,l,d}$$

Factorized expression

$$\tau^0_{\gamma,\delta,w} = \sum_{a \in V} {}^2D^3_{a,w} Y^1_{a,\gamma} Y^{3,*}_{a,\delta} \quad (3r_D r_T^2 N_v) \quad (12900)$$

$$\tau^1_{\gamma,\alpha} = \sum_{a \in V} W^2_{a,\alpha} Y^1_{a,\gamma} \quad (2r_T r_V N_v) \quad (12901)$$

$$\tau^2_{\gamma,\alpha} = \sum_{i \in O} W^1_{i,\alpha} Y^2_{i,\gamma} \quad (2r_T r_V N_o) \quad (12902)$$

$$\tau^3_{\gamma,\alpha} = \sum_{\beta \in B} X_{\beta,\alpha} \tau^1_{\gamma,\beta} \tau^2_{\gamma,\beta} \quad (3r_T r_V^2) \quad (12903)$$

$$\tau^4_{\gamma,\alpha} = \sum_{\delta \in A} Z_{\delta,\gamma} \tau^3_{\delta,\alpha} \quad (2r_T^2 r_V) \quad (12904)$$

$$\tau^5_{\gamma,\alpha} = \sum_{i \in O} W^3_{i,\alpha} Y^4_{i,\gamma} \quad (2r_T r_V N_o) \quad (12905)$$

$$\tau^6_{\gamma,a} = \sum_{\alpha \in B} W^4_{a,\alpha} \tau^4_{\gamma,\alpha} \tau^5_{\gamma,\alpha} \quad (3r_T r_V N_v) \quad (12906)$$

$$\tau^7_{\gamma,\delta} = \sum_{a \in V} Y^3_{a,\delta} \tau^6_{\gamma,a} \quad (2r_T^2 N_v) \quad (12907)$$

$$\tau^8_{\gamma,a} = \sum_{\delta \in A} Y^3_{a,\delta} \tau^7_{\delta,\gamma} \quad (2r_T^2 N_v) \quad (12908)$$

$$\tau^9_{\gamma,\delta,w} = \sum_{a \in V} {}^2D^1_{a,w} Y^{1,*}_{a,\delta} \tau^8_{\gamma,a} \quad (3r_D r_T^2 N_v) \quad (12909)$$

$$\tau_{\gamma,\delta,w}^{10} = \sum_{i \in O} {}^2D_{i,w}^2 Y_{i,\gamma}^4 Y_{i,\delta}^{2,*} \quad (3r_D r_T^2 N_o) \quad (12910)$$

$$\tau_{\gamma,\delta,i}^8 = \sum_{\alpha \in B} W_{i,\alpha}^3 \tau_{\delta,\alpha}^3 \tau_{\gamma,\alpha}^7 \quad (3r_T^2 r_V N_o) \quad (12923)$$

$$\tau_{\gamma,\delta,w}^{11} = \sum_{\epsilon \in A} Z_{\epsilon,\delta}^* \tau_{\gamma,\epsilon,w}^{10} \tau_{\gamma,\epsilon,w}^9 \quad (3r_D r_T^3) \quad (12911)$$

$$\tau_{\gamma,\delta,\epsilon}^9 = \sum_{i \in O} Y_{i,\gamma}^2 \tau_{\delta,\epsilon,i}^8 \quad (2r_T^3 N_o) \quad (12924)$$

$$\tau_{\gamma,\delta,w}^{12} = \sum_{\epsilon \in A} Z_{\gamma,\epsilon} \tau_{\epsilon,\delta,w}^{11} \quad (2r_D r_T^3) \quad (12912)$$

$$\tau_{\gamma,\delta,i}^{10} = \sum_{\epsilon \in A} Z_{\gamma,\epsilon} Y_{i,\epsilon}^4 \tau_{\gamma,\delta,\epsilon}^9 \quad (3r_T^3 N_o) \quad (12925)$$

$${}^2R_{i,\gamma}^4 \leftarrow - \sum_{\delta \in A} \sum_{w \in D} \frac{1}{2} {}^2D_{i,w}^4 Y_{i,\delta}^2 \tau_{\delta,\gamma,w}^0 \tau_{\delta,\gamma,w}^{12} \quad (4r_D r_T^2 N_o) \quad (12913)$$

$$\tau_{\gamma,\delta,w,i}^{11} = \sum_{\epsilon \in A} \tau_{\gamma,\epsilon,i}^{10} \tau_{\epsilon,\delta,w}^2 \quad (2r_D r_T^3 N_o) \quad (12926)$$

Raw expression

$$\tau_{\gamma,\delta,w}^{12} = \sum_{a \in V} {}^2D_{a,w}^3 Y_{a,\gamma}^1 Y_{a,\delta}^{3,*} \quad (3r_D r_T^2 N_v) \quad (12927)$$

$${}^2R_{j,\zeta}^4 \leftarrow - \sum_{\gamma \in A} \sum_{i \in O} \sum_{k \in O} \sum_{l \in O} \sum_{a \in V} \sum_{b \in V} \sum_{c \in V} \sum_{d \in V} \frac{1}{2} \quad (12914)$$

$$Y_{a,\gamma}^{1,*} Y_{i,\gamma}^{2,*} Z_{\gamma,\zeta}^* Y_{b,\zeta}^{3,*} {}^2D_{a,i,b,j}^{a,i,b,j} {}^2T_{b,k,a,i} {}^2T_{c,l,d,j} V_{k,d,l,c}$$

$$\tau_{\gamma,w,i}^{13} = \sum_{\delta \in A} \tau_{\delta,\gamma,w}^{12} \tau_{\delta,\gamma,w,i}^{11} \quad (2r_D r_T^2 N_o) \quad (12928)$$

Factorized expression

$${}^2R_{i,\gamma}^4 \leftarrow - \sum_{w \in D} \frac{1}{2} {}^2D_{i,w}^4 \tau_{\gamma,w,i}^{13} \quad (2r_D r_T N_o) \quad (12929)$$

$$\tau_{\gamma,\delta,w}^0 = \sum_{a \in V} {}^2D_{a,w}^1 Y_{a,\gamma}^3 Y_{a,\delta}^{1,*} \quad (3r_D r_T^2 N_v) \quad (12915)$$

Raw expression

$$\tau_{\gamma,\delta,w}^1 = \sum_{i \in O} {}^2D_{i,w}^2 Y_{i,\gamma}^4 Y_{i,\delta}^{2,*} \quad (3r_D r_T^2 N_o) \quad (12916)$$

$${}^2R_{j,\zeta}^4 \leftarrow - \sum_{\gamma \in A} \sum_{i \in O} \sum_{k \in O} \sum_{l \in O} \sum_{a \in V} \sum_{b \in V} \sum_{c \in V} \sum_{d \in V} \frac{1}{2} \quad (12930)$$

$$Y_{a,\gamma}^{1,*} Y_{i,\gamma}^{2,*} Z_{\gamma,\zeta}^* Y_{b,\zeta}^{3,*} {}^2D_{a,i,b,j}^{a,i,b,j} {}^2T_{b,k,c,l} {}^2T_{d,j,a,i} V_{k,d,l,c}$$

$$\tau_{\gamma,\delta,w}^2 = \sum_{\epsilon \in A} Z_{\epsilon,\delta}^* \tau_{\gamma,\epsilon,w}^0 \tau_{\gamma,\epsilon,w}^1 \quad (3r_D r_T^3) \quad (12917)$$

Factorized expression

$$\tau_{\gamma,\alpha}^3 = \sum_{a \in V} W_{a,\alpha}^4 Y_{a,\gamma}^3 \quad (2r_T r_V N_v) \quad (12918)$$

$$\tau_{\gamma,\delta,w}^0 = \sum_{a \in V} {}^2D_{a,w}^1 Y_{a,\gamma}^3 Y_{a,\delta}^{1,*} \quad (3r_D r_T^2 N_v) \quad (12931)$$

$$\tau_{\gamma,\alpha}^4 = \sum_{a \in V} W_{a,\alpha}^2 Y_{a,\gamma}^1 \quad (2r_T r_V N_v) \quad (12919)$$

$$\tau_{\gamma,\delta,w}^1 = \sum_{i \in O} {}^2D_{i,w}^2 Y_{i,\gamma}^4 Y_{i,\delta}^{2,*} \quad (3r_D r_T^2 N_o) \quad (12932)$$

$$\tau_{\gamma,\alpha}^5 = \sum_{i \in O} W_{i,\alpha}^1 Y_{i,\gamma}^2 \quad (2r_T r_V N_o) \quad (12920)$$

$$\tau_{\gamma,\delta,w}^2 = \sum_{\epsilon \in A} Z_{\epsilon,\delta}^* \tau_{\gamma,\epsilon,w}^0 \tau_{\gamma,\epsilon,w}^1 \quad (3r_D r_T^3) \quad (12933)$$

$$\tau_{\gamma,\alpha}^6 = \sum_{\beta \in B} X_{\beta,\alpha} \tau_{\gamma,\beta}^4 \tau_{\gamma,\beta}^5 \quad (3r_T r_V^2) \quad (12921)$$

$$\tau_{\gamma,\alpha}^3 = \sum_{a \in V} W_{a,\alpha}^2 Y_{a,\gamma}^3 \quad (2r_T r_V N_v) \quad (12934)$$

$$\tau_{\gamma,\alpha}^7 = \sum_{\delta \in A} Z_{\delta,\gamma} \tau_{\delta,\alpha}^6 \quad (2r_T^2 r_V) \quad (12922)$$

$$\tau_{\gamma,\alpha,i}^4 = \sum_{\beta \in B} W_{i,\beta}^1 X_{\beta,\alpha} \tau_{\gamma,\beta}^3 \quad (3r_T r_V^2 N_o) \quad (12935)$$

$$\tau^5_{\gamma,\alpha} = \sum_{i \in O} W^3_{i,\alpha} Y^4_{i,\gamma} \quad (2r_T r_V N_o) \quad (12936)$$

$$\tau^2_{\gamma,\alpha} = \sum_{a \in V} W^4_{a,\alpha} Y^1_{a,\gamma} \quad (2r_T r_V N_v) \quad (12948)$$

$$\tau^6_{\gamma,\alpha} = \sum_{a \in V} W^4_{a,\alpha} Y^1_{a,\gamma} \quad (2r_T r_V N_v) \quad (12937)$$

$$\tau^3_{\gamma,\alpha} = \sum_{i \in O} W^3_{i,\alpha} Y^2_{i,\gamma} \quad (2r_T r_V N_o) \quad (12949)$$

$$\tau^7_{\gamma,\delta,i} = \sum_{\alpha \in B} \tau^5_{\delta,\alpha} \tau^6_{\gamma,\alpha} \tau^4_{\delta,\alpha,i} \quad (3r_T^2 r_V N_o) \quad (12938)$$

$$\tau^4_{\gamma,\alpha} = \sum_{\beta \in B} X_{\alpha,\beta} \tau^2_{\gamma,\beta} \tau^3_{\gamma,\beta} \quad (3r_T r_V^2) \quad (12950)$$

$$\tau^8_{\gamma,\delta} = \sum_{i \in O} Y^2_{i,\gamma} \tau^7_{\gamma,\delta,i} \quad (2r_T^2 N_o) \quad (12939)$$

$$\tau^5_{\gamma,\alpha} = \sum_{\delta \in A} Z_{\delta,\gamma} \tau^4_{\delta,\alpha} \quad (2r_T^2 r_V) \quad (12951)$$

$$\tau^9_{\gamma,\delta} = \sum_{\epsilon \in A} Z_{\delta,\epsilon} \tau^8_{\gamma,\epsilon} \quad (2r_T^3) \quad (12940)$$

$$\tau^6_{\gamma,\alpha} = \sum_{a \in V} W^2_{a,\alpha} Y^3_{a,\gamma} \quad (2r_T r_V N_v) \quad (12952)$$

$$\tau^{10}_{\gamma,\delta} = \sum_{\epsilon \in A} Z_{\delta,\epsilon} \tau^9_{\epsilon,\gamma} \quad (2r_T^3) \quad (12941)$$

$$\tau^7_{\gamma,i} = \sum_{\alpha \in B} W^1_{i,\alpha} \tau^5_{\gamma,\alpha} \tau^6_{\gamma,\alpha} \quad (3r_T r_V N_o) \quad (12953)$$

$$\tau^{11}_{\gamma,\delta,w} = \sum_{\epsilon \in A} \tau^{10}_{\gamma,\epsilon} \tau^2_{\epsilon,\delta,w} \quad (2r_D r_T^3) \quad (12942)$$

$$\tau^8_{i,j} = \sum_{\gamma \in A} Y^4_{j,\gamma} \tau^7_{\gamma,i} \quad (2r_T N_o^2) \quad (12954)$$

$$\tau^{12}_{\gamma,\delta,w} = \sum_{a \in V} {}^2D^3_{a,w} Y^1_{a,\gamma} Y^{3,*}_{a,\delta} \quad (3r_D r_T^2 N_v) \quad (12943)$$

$$\tau^9_{\gamma,i} = \sum_{j \in O} Y^4_{j,\gamma} \tau^8_{j,i} \quad (2r_T N_o^2) \quad (12955)$$

$$\tau^{10}_{\gamma,\delta,w} = \sum_{i \in O} {}^2D^2_{i,w} Y^{2,*}_{i,\delta} \tau^9_{\gamma,i} \quad (3r_D r_T^2 N_o) \quad (12956)$$

$${}^2R^4_{i,\gamma} \leftarrow - \sum_{\delta \in A} \sum_{w \in D} \frac{1}{2} {}^2D^4_{i,w} Y^2_{i,\delta} \tau^{11}_{\delta,\gamma,w} \tau^{12}_{\delta,\gamma,w} \quad (4r_D r_T^2 N_o) \quad (12944)$$

$$\tau^{11}_{\gamma,\delta,w} = \sum_{\epsilon \in A} Z^*_{\epsilon,\delta} \tau^1_{\gamma,\epsilon,w} \tau^{10}_{\gamma,\epsilon,w} \quad (3r_D r_T^3) \quad (12957)$$

Raw expression

$${}^2R^4_{j,\zeta} \leftarrow - \sum_{\gamma \in A} \sum_{i \in O} \sum_{k \in O} \sum_{l \in O} \sum_{a \in V} \sum_{b \in V} \sum_{c \in V} \sum_{d \in V} \frac{1}{2} Y^{1,*}_{a,\gamma} Y^{2,*}_{i,\gamma} Z^*_{\gamma,\zeta} Y^{3,*}_{b,\zeta} {}^2D^{a,i,b,j} {}^2T_{b,l,d,j} {}^2T_{c,k,a,i} V_{k,c,l,d} \quad (12945)$$

$$\tau^{12}_{\gamma,\delta,w} = \sum_{\epsilon \in A} Z_{\gamma,\epsilon} \tau^{11}_{\epsilon,\delta,w} \quad (2r_D r_T^3) \quad (12958)$$

$${}^2R^4_{i,\gamma} \leftarrow - \sum_{\delta \in A} \sum_{w \in D} \frac{1}{2} {}^2D^4_{i,w} Y^2_{i,\delta} \tau^0_{\delta,\gamma,w} \tau^{12}_{\delta,\gamma,w} \quad (4r_D r_T^2 N_o) \quad (12959)$$

Factorized expression

$$\tau^0_{\gamma,\delta,w} = \sum_{a \in V} {}^2D^3_{a,w} Y^1_{a,\gamma} Y^{3,*}_{a,\delta} \quad (3r_D r_T^2 N_v) \quad (12946)$$

Raw expression

$${}^2R^4_{j,\zeta} \leftarrow - \sum_{\gamma \in A} \sum_{i \in O} \sum_{k \in O} \sum_{l \in O} \sum_{a \in V} \sum_{b \in V} \sum_{c \in V} \sum_{d \in V} \frac{1}{2} Y^{1,*}_{a,\gamma} Y^{2,*}_{i,\gamma} Z^*_{\gamma,\zeta} Y^{3,*}_{b,\zeta} {}^2D^{a,i,b,j} {}^2T_{c,i,a,k} {}^2T_{d,l,b,j} V_{k,c,l,d} \quad (12960)$$

$$\tau^1_{\gamma,\delta,w} = \sum_{a \in V} {}^2D^1_{a,w} Y^3_{a,\gamma} Y^{1,*}_{a,\delta} \quad (3r_D r_T^2 N_v) \quad (12947)$$

Factorized expression

$$\tau_{\gamma,\delta,w}^0 = \sum_{a \in V} {}^2D_{a,w}^1 Y_{a,\gamma}^3 Y_{a,\delta}^{1,*} \quad (3r_D r_T^2 N_v) \quad (12961)$$

$$\tau_{\gamma,\alpha}^1 = \sum_{a \in V} W_{a,\alpha}^2 Y_{a,\gamma}^1 \quad (2r_T r_V N_v) \quad (12962)$$

$$\tau_{\gamma,\alpha}^2 = \sum_{a \in V} W_{a,\alpha}^4 Y_{a,\gamma}^1 \quad (2r_T r_V N_v) \quad (12963)$$

$$\tau_{\gamma,\alpha}^3 = \sum_{i \in O} W_{i,\alpha}^3 Y_{i,\gamma}^2 \quad (2r_T r_V N_o) \quad (12964)$$

$$\tau_{\gamma,\alpha}^4 = \sum_{\beta \in B} X_{\alpha,\beta} \tau_{\gamma,\beta}^2 \tau_{\gamma,\beta}^3 \quad (3r_T r_V^2) \quad (12965)$$

$$\tau_{\gamma,\alpha}^5 = \sum_{\delta \in A} Z_{\delta,\gamma} \tau_{\delta,\alpha}^4 \quad (2r_T^2 r_V) \quad (12966)$$

$$\tau_{\gamma,\delta,i}^6 = \sum_{\alpha \in B} W_{i,\alpha}^1 \tau_{\gamma,\alpha}^1 \tau_{\delta,\alpha}^5 \quad (3r_T^2 r_V N_o) \quad (12967)$$

$$\tau_{\gamma,\delta,\epsilon}^7 = \sum_{i \in O} Z_{\gamma,\delta} Y_{i,\delta}^4 \tau_{\gamma,\epsilon,i}^6 \quad (3r_T^3 N_o) \quad (12968)$$

$$\tau_{\gamma,\delta,i}^8 = \sum_{\epsilon \in A} Y_{i,\epsilon}^2 \tau_{\epsilon,\gamma,\delta}^7 \quad (2r_T^3 N_o) \quad (12969)$$

$$\tau_{\gamma,\delta,w}^9 = \sum_{\epsilon \in A} \sum_{i \in O} {}^2D_{i,w}^2 Y_{i,\delta}^{2,*} \tau_{\epsilon,\delta,w}^0 \tau_{\epsilon,\gamma,i}^8 \quad (4r_D r_T^3 N_o) \quad (12970)$$

$$\tau_{\gamma,\delta,w}^{10} = \sum_{\epsilon \in A} Z_{\epsilon,\delta}^* \tau_{\gamma,\epsilon,w}^9 \quad (2r_D r_T^3) \quad (12971)$$

$$\tau_{\gamma,\delta,w}^{11} = \sum_{a \in V} {}^2D_{a,w}^3 Y_{a,\gamma}^3 Y_{a,\delta}^{3,*} \quad (3r_D r_T^2 N_v) \quad (12972)$$

$${}^2R_{i,\gamma}^4 \leftarrow - \sum_{\delta \in A} \sum_{w \in D} \frac{1}{2} {}^2D_{i,w}^4 Y_{i,\delta}^4 \tau_{\delta,\gamma,w}^{10} \tau_{\delta,\gamma,w}^{11} \quad (4r_D r_T^2 N_o) \quad (12973)$$

Raw expression

$${}^2R_{j,\zeta}^4 \leftarrow - \sum_{\gamma \in A} \sum_{i \in O} \sum_{k \in O} \sum_{l \in O} \sum_{a \in V} \sum_{b \in V} \sum_{c \in V} \sum_{d \in V} \frac{1}{2} Y_{a,\gamma}^{1,*} Y_{i,\gamma}^{2,*} Z_{\gamma,\zeta}^* Y_{b,\zeta}^{3,*} {}^2D_{a,i,b,j} {}^2T_{c,k,a,i} {}^2T_{d,j,b,l} V_{k,c,l,d} \quad (12974)$$

Factorized expression

$$\tau_{\gamma,\alpha}^0 = \sum_{a \in V} W_{a,\alpha}^2 Y_{a,\gamma}^1 \quad (2r_T r_V N_v) \quad (12975)$$

$$\tau_{\gamma,\alpha}^1 = \sum_{i \in O} W_{i,\alpha}^1 Y_{i,\gamma}^2 \quad (2r_T r_V N_o) \quad (12976)$$

$$\tau_{\gamma,\alpha}^2 = \sum_{\beta \in B} X_{\beta,\alpha} \tau_{\gamma,\beta}^0 \tau_{\gamma,\beta}^1 \quad (3r_T r_V^2) \quad (12977)$$

$$\tau_{\gamma,\alpha}^3 = \sum_{\delta \in A} Z_{\delta,\gamma} \tau_{\delta,\alpha}^2 \quad (2r_T^2 r_V) \quad (12978)$$

$$\tau_{\gamma,\alpha}^4 = \sum_{i \in O} W_{i,\alpha}^3 Y_{i,\gamma}^4 \quad (2r_T r_V N_o) \quad (12979)$$

$$\tau_{\gamma,a}^5 = \sum_{\alpha \in B} W_{a,\alpha}^4 \tau_{\gamma,\alpha}^3 \tau_{\gamma,\alpha}^4 \quad (3r_T r_V N_v) \quad (12980)$$

$$\tau_{\gamma,\delta}^6 = \sum_{a \in V} Y_{a,\gamma}^1 \tau_{\delta,a}^5 \quad (2r_T^2 N_v) \quad (12981)$$

$$\tau_{\gamma,a}^7 = \sum_{\delta \in A} Y_{a,\delta}^3 \tau_{\gamma,\delta}^6 \quad (2r_T^2 N_v) \quad (12982)$$

$$\tau_{\gamma,\delta,w}^8 = \sum_{a \in V} {}^2D_{a,w}^3 Y_{a,\delta}^{3,*} \tau_{\gamma,a}^7 \quad (3r_D r_T^2 N_v) \quad (12983)$$

$$\tau_{\gamma,\delta,w}^9 = \sum_{a \in V} {}^2D_{a,w}^1 Y_{a,\gamma}^3 Y_{a,\delta}^{1,*} \quad (3r_D r_T^2 N_v) \quad (12984)$$

$$\tau_{\gamma,\delta,w}^{10} = \sum_{i \in O} {}^2D_{i,w}^2 Y_{i,\gamma}^4 Y_{i,\delta}^{2,*} \quad (3r_D r_T^2 N_o) \quad (12985)$$

$$\tau_{\gamma,\delta,w}^{11} = \sum_{\epsilon \in A} Z_{\epsilon,\delta}^* \tau_{\gamma,\epsilon,w}^{10} \tau_{\gamma,\epsilon,w}^9 \quad (3r_D r_T^3) \quad (12986)$$



$$\tau^{12}_{\gamma,\delta,w} = \sum_{\epsilon \in A} Z_{\gamma,\epsilon} \tau^{11}_{\epsilon,\delta,w} \quad (2r_D r_T^3) \quad (12987)$$

$$\tau^{10}_{\gamma,\delta,i} = \sum_{\epsilon \in A} Y^2_{i,\epsilon} \tau^9_{\epsilon,\gamma,\delta} \quad (2r_T^3 N_o) \quad (13000)$$

$${}^2R^4_{i,\gamma} \leftarrow - \sum_{\delta \in A} \sum_{w \in D} \frac{1}{2} {}^2D^4_{i,w} Y^2_{i,\delta} \tau^{12}_{\delta,\gamma,w} \tau^8_{\delta,\gamma,w} \quad (4r_D r_T^2 N_o) \quad (12988)$$

$$\tau^{11}_{\gamma,\delta,w} = \sum_{a \in V} {}^2D^3_{a,w} Y^3_{a,\gamma} Y^{3,*}_{a,\delta} \quad (3r_D r_T^2 N_v) \quad (13001)$$

Raw expression

$${}^2R^4_{j,\zeta} \leftarrow - \sum_{\gamma \in A} \sum_{i \in O} \sum_{k \in O} \sum_{l \in O} \sum_{a \in V} \sum_{b \in V} \sum_{c \in V} \sum_{d \in V} \frac{1}{2} \quad (12989)$$

$$Y^{1,*}_{a,\gamma} Y^{2,*}_{i,\gamma} Z^*_{\gamma,\zeta} Y^{3,*}_{b,\zeta} \\ {}^2D^{a,i,b,j}_{c,k,a,i} {}^2T_{c,k,a,i} {}^2T_{d,l,b,j} V_{k,d,l,c}$$

$$\tau^{12}_{\gamma,\delta,w,i} = \sum_{\epsilon \in A} \tau^{10}_{\epsilon,\gamma,i} \tau^{11}_{\epsilon,\delta,w} \quad (2r_D r_T^3 N_o) \quad (13002)$$

$$\tau^{13}_{\gamma,w,i} = \sum_{\delta \in A} \tau^2_{\delta,\gamma,w} \tau^{12}_{\delta,\gamma,w,i} \quad (2r_D r_T^2 N_o) \quad (13003)$$

Factorized expression

$$\tau^0_{\gamma,\delta,w} = \sum_{a \in V} {}^2D^1_{a,w} Y^3_{a,\gamma} Y^{1,*}_{a,\delta} \quad (3r_D r_T^2 N_v) \quad (12990)$$

$$\tau^1_{\gamma,\delta,w} = \sum_{i \in O} {}^2D^2_{i,w} Y^4_{i,\gamma} Y^{2,*}_{i,\delta} \quad (3r_D r_T^2 N_o) \quad (12991)$$

$$\tau^2_{\gamma,\delta,w} = \sum_{\epsilon \in A} Z^*_{\epsilon,\delta} \tau^0_{\gamma,\epsilon,w} \tau^1_{\gamma,\epsilon,w} \quad (3r_D r_T^3) \quad (12992)$$

$$\tau^3_{\gamma,\alpha} = \sum_{a \in V} W^2_{a,\alpha} Y^1_{a,\gamma} \quad (2r_T r_V N_v) \quad (12993)$$

$$\tau^4_{\gamma,\alpha} = \sum_{i \in O} W^1_{i,\alpha} Y^2_{i,\gamma} \quad (2r_T r_V N_o) \quad (12994)$$

$$\tau^5_{\gamma,\alpha} = \sum_{\beta \in B} X_{\beta,\alpha} \tau^3_{\gamma,\beta} \tau^4_{\gamma,\beta} \quad (3r_T r_V^2) \quad (12995)$$

$$\tau^6_{\gamma,\alpha} = \sum_{\delta \in A} Z_{\delta,\gamma} \tau^5_{\delta,\alpha} \quad (2r_T^2 r_V) \quad (12996)$$

$$\tau^7_{\gamma,\alpha} = \sum_{a \in V} W^4_{a,\alpha} Y^1_{a,\gamma} \quad (2r_T r_V N_v) \quad (12997)$$

$$\tau^8_{\gamma,\delta,i} = \sum_{\alpha \in B} W^3_{i,\alpha} \tau^6_{\delta,\alpha} \tau^7_{\gamma,\alpha} \quad (3r_T^2 r_V N_o) \quad (12998)$$

$$\tau^9_{\gamma,\delta,\epsilon} = \sum_{i \in O} Z_{\gamma,\delta} Y^4_{i,\delta} \tau^8_{\gamma,\epsilon,i} \quad (3r_T^3 N_o) \quad (12999)$$

$${}^2R^4_{i,\gamma} \leftarrow - \sum_{w \in D} \frac{1}{2} {}^2D^4_{i,w} \tau^{13}_{\gamma,w,i} \quad (2r_D r_T N_o) \quad (13004)$$

Raw expression

$${}^2R^4_{j,\zeta} \leftarrow - \sum_{\gamma \in A} \sum_{i \in O} \sum_{k \in O} \sum_{l \in O} \sum_{a \in V} \sum_{b \in V} \sum_{c \in V} \sum_{d \in V} \frac{1}{2} \quad (13005)$$

$$Y^{1,*}_{a,\gamma} Y^{2,*}_{i,\gamma} Z^*_{\gamma,\zeta} Y^{3,*}_{b,\zeta} \\ {}^2D^{a,i,b,j}_{c,k,a,l} {}^2T_{c,k,a,l} {}^2T_{d,i,b,j} V_{k,c,l,d}$$

Factorized expression

$$\tau^0_{\gamma,\delta,w} = \sum_{a \in V} {}^2D^3_{a,w} Y^3_{a,\gamma} Y^{3,*}_{a,\delta} \quad (3r_D r_T^2 N_v) \quad (13006)$$

$$\tau^1_{\gamma,\delta,w} = \sum_{i \in O} {}^2D^2_{i,w} Y^2_{i,\gamma} Y^{2,*}_{i,\delta} \quad (3r_D r_T^2 N_o) \quad (13007)$$

$$\tau^2_{\gamma,\alpha} = \sum_{a \in V} W^2_{a,\alpha} Y^1_{a,\gamma} \quad (2r_T r_V N_v) \quad (13008)$$

$$\tau^3_{\gamma,\alpha} = \sum_{i \in O} W^1_{i,\alpha} Y^2_{i,\gamma} \quad (2r_T r_V N_o) \quad (13009)$$

$$\tau^4_{\gamma,\alpha} = \sum_{\beta \in B} X_{\beta,\alpha} \tau^2_{\gamma,\beta} \tau^3_{\gamma,\beta} \quad (3r_T r_V^2) \quad (13010)$$

$$\tau^5_{\gamma,\alpha} = \sum_{\delta \in A} Z_{\delta,\gamma} \tau^4_{\delta,\alpha} \quad (2r_T^2 r_V) \quad (13011)$$

$$\tau^6_{\gamma,\alpha} = \sum_{i \in O} W^3_{i,\alpha} Y^4_{i,\gamma} \quad (2r_T r_V N_o) \quad (13012)$$

$$\tau_{\gamma,a}^7 = \sum_{\alpha \in B} W_{a,\alpha}^4 \tau_{\gamma,\alpha}^5 \tau_{\gamma,\alpha}^6 \quad (3r_T r_V N_v) \quad (13013)$$

$$\tau_{\gamma,\alpha}^5 = \sum_{i \in O} W_{i,\alpha}^3 Y_{i,\gamma}^2 \quad (2r_T r_V N_o) \quad (13026)$$

$$\tau_{\gamma,\delta}^8 = \sum_{a \in V} Y_{a,\gamma}^1 \tau_{\delta,a}^7 \quad (2r_T^2 N_v) \quad (13014)$$

$$\tau_{\gamma,\alpha}^6 = \sum_{a \in V} W_{a,\alpha}^4 Y_{a,\gamma}^1 \quad (2r_T r_V N_v) \quad (13027)$$

$$\tau_{\gamma,a}^9 = \sum_{\delta \in A} Y_{a,\delta}^3 \tau_{\gamma,\delta}^8 \quad (2r_T^2 N_v) \quad (13015)$$

$$\tau_{\gamma,\delta,i}^7 = \sum_{\alpha \in B} \tau_{\gamma,\alpha}^5 \tau_{\delta,\alpha}^6 \tau_{\gamma,\alpha,i}^4 \quad (3r_T^2 r_V N_o) \quad (13028)$$

$$\tau_{\gamma,\delta,w}^{10} = \sum_{a \in V} {}^2D_{a,w}^1 Y_{a,w}^{1,*} \tau_{\gamma,a}^9 \quad (3r_D r_T^2 N_v) \quad (13016)$$

$$\tau_{\gamma,\delta}^8 = \sum_{i \in O} Y_{i,\delta}^2 \tau_{\gamma,\delta,i}^7 \quad (2r_T^2 N_o) \quad (13029)$$

$$\tau_{\gamma,\delta,w}^{11} = \sum_{\epsilon \in A} Z_{\epsilon,\delta}^* \tau_{\gamma,\epsilon,w}^1 \tau_{\gamma,\epsilon,w}^{10} \quad (3r_D r_T^3) \quad (13017)$$

$$\tau_{\gamma,\delta}^9 = \sum_{\epsilon \in A} Z_{\epsilon,\delta} \tau_{\gamma,\epsilon}^8 \quad (2r_T^3) \quad (13030)$$

$$\tau_{\gamma,\delta,w}^{12} = \sum_{\epsilon \in A} Z_{\epsilon,\gamma} \tau_{\epsilon,\delta,w}^{11} \quad (2r_D r_T^3) \quad (13018)$$

$$\tau_{\gamma,\delta}^{10} = \sum_{\epsilon \in A} Z_{\epsilon,\gamma} \tau_{\epsilon,\delta}^9 \quad (2r_T^3) \quad (13031)$$

$${}^2R_{i,\gamma}^4 \leftarrow - \sum_{\delta \in A} \sum_{w \in D} \frac{1}{2} {}^2D_{i,w}^4 Y_{i,\delta}^4 \tau_{\delta,\gamma,w}^0 \tau_{\delta,\gamma,w}^{12} \quad (4r_D r_T^2 N_o) \quad (13019)$$

$$\tau_{\gamma,\delta,w}^{11} = \sum_{\epsilon \in A} \tau_{\gamma,\epsilon}^{10} \tau_{\epsilon,\delta,w}^2 \quad (2r_D r_T^3) \quad (13032)$$

$$\tau_{\gamma,\delta,w}^{12} = \sum_{a \in V} {}^2D_{a,w}^3 Y_{a,\gamma}^3 Y_{a,\delta}^{3,*} \quad (3r_D r_T^2 N_v) \quad (13033)$$

Raw expression

$${}^2R_{j,\zeta}^4 \leftarrow - \sum_{\gamma \in A} \sum_{i \in O} \sum_{k \in O} \sum_{l \in O} \sum_{a \in V} \sum_{b \in V} \sum_{c \in V} \sum_{d \in V} \frac{1}{2} \quad (13020)$$

$$Y_{a,\gamma}^{1,*} Y_{i,\gamma}^{2,*} Z_{\gamma,\zeta}^* Y_{b,\zeta}^{3,*} {}^2D_{a,i,b,j} {}^2T_{c,k,b,l} {}^2T_{d,j,a,i} V_{k,c,l,d}$$

$${}^2R_{i,\gamma}^4 \leftarrow - \sum_{\delta \in A} \sum_{w \in D} \frac{1}{2} {}^2D_{i,w}^4 Y_{i,\delta}^4 \tau_{\delta,\gamma,w}^{11} \tau_{\delta,\gamma,w}^{12} \quad (4r_D r_T^2 N_o) \quad (13034)$$

Factorized expression

$$\tau_{\gamma,\delta,w}^0 = \sum_{a \in V} {}^2D_{a,w}^1 Y_{a,\gamma}^3 Y_{a,\delta}^{1,*} \quad (3r_D r_T^2 N_v) \quad (13021)$$

Raw expression

$${}^2R_{j,\zeta}^4 \leftarrow \sum_{\gamma \in A} \sum_{i \in O} \sum_{k \in O} \sum_{l \in O} \sum_{a \in V} \sum_{b \in V} \sum_{c \in V} \sum_{d \in V} \frac{1}{4} \quad (13035)$$

$$Y_{a,\gamma}^{1,*} Y_{i,\gamma}^{2,*} Z_{\gamma,\zeta}^* Y_{b,\zeta}^{3,*} {}^2D_{a,i,b,j} {}^2T_{a,i,b,k} {}^2T_{c,j,d,l} V_{k,d,l,c}$$

$$\tau_{\gamma,\delta,w}^1 = \sum_{i \in O} {}^2D_{i,w}^2 Y_{i,\gamma}^4 Y_{i,\delta}^{2,*} \quad (3r_D r_T^2 N_o) \quad (13022)$$

Factorized expression

$$\tau_{\gamma,\delta,w}^2 = \sum_{\epsilon \in A} Z_{\epsilon,\delta}^* \tau_{\gamma,\epsilon,w}^0 \tau_{\gamma,\epsilon,w}^1 \quad (3r_D r_T^3) \quad (13023)$$

$$\tau_{\gamma,\delta,w}^0 = \sum_{a \in V} {}^2D_{a,w}^1 Y_{a,\gamma}^1 Y_{a,\delta}^{1,*} \quad (3r_D r_T^2 N_v) \quad (13036)$$

$$\tau_{\gamma,\alpha}^3 = \sum_{a \in V} W_{a,\alpha}^2 Y_{a,\gamma}^1 \quad (2r_T r_V N_v) \quad (13024)$$

$$\tau_{\gamma,\delta,w}^1 = \sum_{i \in O} {}^2D_{i,w}^2 Y_{i,\gamma}^2 Y_{i,\delta}^{2,*} \quad (3r_D r_T^2 N_o) \quad (13037)$$

$$\tau_{\gamma,\alpha,i}^4 = \sum_{\beta \in B} W_{i,\beta}^1 X_{\beta,\alpha} \tau_{\gamma,\beta}^3 \quad (3r_T r_V^2 N_o) \quad (13025)$$

$$\tau_{\gamma,\delta,w}^2 = \sum_{\epsilon \in A} Z_{\epsilon,\delta}^* \tau_{\gamma,\epsilon,w}^0 \tau_{\gamma,\epsilon,w}^1 \quad (3r_D r_T^3) \quad (13038)$$

$$\tau^3_{\gamma,\delta,w} = \sum_{\epsilon \in A} Z_{\epsilon,\gamma} \tau^2_{\epsilon,\delta,w} \quad (2r_D r_T^3) \quad (13039)$$

$$\tau^1_{\gamma,\delta,w} = \sum_{a \in V} {}^2D^1_{a,w} Y^1_{a,\gamma} Y^{1,*}_{a,\delta} \quad (3r_D r_T^2 N_v) \quad (13051)$$

$$\tau^4_{\gamma,\alpha} = \sum_{a \in V} W^2_{a,\alpha} Y^3_{a,\gamma} \quad (2r_T r_V N_v) \quad (13040)$$

$$\tau^2_{\gamma,\delta,w} = \sum_{i \in O} {}^2D^2_{i,w} Y^2_{i,\gamma} Y^{2,*}_{i,\delta} \quad (3r_D r_T^2 N_o) \quad (13052)$$

$$\tau^5_{\gamma,\alpha,i} = \sum_{\beta \in B} W^1_{i,\beta} X_{\beta,\alpha} \tau^4_{\gamma,\beta} \quad (3r_T r_V^2 N_o) \quad (13041)$$

$$\tau^3_{\gamma,\delta,w} = \sum_{\epsilon \in A} Z^*_{\epsilon,\delta} \tau^1_{\gamma,\epsilon,w} \tau^2_{\gamma,\epsilon,w} \quad (3r_D r_T^3) \quad (13053)$$

$$\tau^6_{\gamma,\alpha} = \sum_{i \in O} W^3_{i,\alpha} Y^4_{i,\gamma} \quad (2r_T r_V N_o) \quad (13042)$$

$$\tau^4_{\gamma,\delta,w} = \sum_{\epsilon \in A} Z_{\epsilon,\gamma} \tau^3_{\epsilon,\delta,w} \quad (2r_D r_T^3) \quad (13054)$$

$$\tau^7_{\gamma,\alpha} = \sum_{\delta \in A} \sum_{i \in O} Y^2_{i,\gamma} Z_{\gamma,\delta} \tau^6_{\delta,\alpha} \tau^5_{\delta,\alpha,i} \quad (4r_T^2 r_V N_o) \quad (13043)$$

$$\tau^5_{\gamma,\alpha} = \sum_{a \in V} W^4_{a,\alpha} Y^3_{a,\gamma} \quad (2r_T r_V N_v) \quad (13055)$$

$$\tau^8_{\gamma,a} = \sum_{\alpha \in B} W^4_{a,\alpha} \tau^7_{\gamma,\alpha} \quad (2r_T r_V N_v) \quad (13044)$$

$$\tau^6_{\gamma,\alpha,i} = \sum_{\beta \in B} X_{\alpha,\beta} W^3_{i,\beta} \tau^5_{\gamma,\beta} \quad (3r_T r_V^2 N_o) \quad (13056)$$

$$\tau^9_{\gamma,\delta} = \sum_{a \in V} Y^3_{a,\delta} \tau^8_{\gamma,a} \quad (2r_T^2 N_v) \quad (13045)$$

$$\tau^7_{\gamma,\alpha} = \sum_{i \in O} W^1_{i,\alpha} Y^4_{i,\gamma} \quad (2r_T r_V N_o) \quad (13057)$$

$$\tau^{10}_{\gamma,a} = \sum_{\delta \in A} Y^1_{a,\delta} \tau^9_{\delta,\gamma} \quad (2r_T^2 N_v) \quad (13046)$$

$$\tau^8_{\gamma,\alpha} = \sum_{a \in V} W^2_{a,\alpha} Y^3_{a,\gamma} \quad (2r_T r_V N_v) \quad (13058)$$

$$\tau^{11}_{\gamma,\delta,w} = \sum_{a \in V} {}^2D^3_{a,w} Y^{3,*}_{a,\delta} \tau^{10}_{\gamma,a} \quad (3r_D r_T^2 N_v) \quad (13047)$$

$$\tau^9_{\gamma,\delta,i} = \sum_{\alpha \in B} \tau^7_{\gamma,\alpha} \tau^8_{\delta,\alpha} \tau^6_{\gamma,\alpha,i} \quad (3r_T^2 r_V N_o) \quad (13059)$$

$${}^2R^4_{i,\gamma} \leftarrow \sum_{\delta \in A} \sum_{w \in D} \frac{1}{4} {}^2D^4_{i,w} Y^4_{i,\delta} \tau^{11}_{\delta,\gamma,w} \tau^3_{\delta,\gamma,w} \quad (4r_D r_T^2 N_o) \quad (13048)$$

$$\tau^{10}_{\gamma,\delta,\epsilon} = \sum_{i \in O} Y^2_{i,\gamma} Z_{\gamma,\delta} \tau^9_{\epsilon,\delta,i} \quad (3r_T^3 N_o) \quad (13060)$$

$$\tau^{11}_{\gamma,\delta,i} = \sum_{\epsilon \in A} Y^4_{i,\epsilon} \tau^{10}_{\gamma,\epsilon,\delta} \quad (2r_T^3 N_o) \quad (13061)$$

Raw expression

$${}^2R^4_{j,\zeta} \leftarrow \sum_{\gamma \in A} \sum_{i \in O} \sum_{k \in O} \sum_{l \in O} \sum_{a \in V} \sum_{b \in V} \sum_{c \in V} \sum_{d \in V} \frac{1}{4} Y^{1,*}_{a,\gamma} Y^{2,*}_{i,\gamma} Z^*_{\gamma,\zeta} Y^{3,*}_{b,\zeta} {}^2D^{a,i,b,j}_{a,i,b,k} {}^2T_{a,i,b,k} {}^2T_{c,l,d,j} V_{k,c,l,d} \quad (13049)$$

$$\tau^{12}_{\gamma,\delta,w,i} = \sum_{\epsilon \in A} \tau^{11}_{\gamma,\epsilon,i} \tau^4_{\epsilon,\delta,w} \quad (2r_D r_T^3 N_o) \quad (13062)$$

$$\tau^{13}_{\gamma,w,i} = \sum_{\delta \in A} \tau^0_{\delta,\gamma,w} \tau^{12}_{\delta,\gamma,w,i} \quad (2r_D r_T^2 N_o) \quad (13063)$$

Factorized expression

$$\tau^0_{\gamma,\delta,w} = \sum_{a \in V} {}^2D^3_{a,w} Y^1_{a,\gamma} Y^{3,*}_{a,\delta} \quad (3r_D r_T^2 N_v) \quad (13050)$$

$${}^2R^4_{i,\gamma} \leftarrow \sum_{w \in D} \frac{1}{4} {}^2D^4_{i,w} \tau^{13}_{\gamma,w,i} \quad (2r_D r_T N_o) \quad (13064)$$

Raw expression

$${}^2R^4_{j,\zeta} \leftarrow \sum_{\gamma \in A} \sum_{i \in O} \sum_{k \in O} \sum_{l \in O} \sum_{a \in V} \sum_{b \in V} \sum_{c \in V} \sum_{d \in V} \frac{1}{4} \quad (13065)$$

$$Y^{1,*}_{a,\gamma} \quad Y^{2,*}_{i,\gamma} \quad Z^*_{\gamma,\zeta} \quad Y^{3,*}_{b,\zeta}$$

$${}^2D^{a,i,b,j} \quad {}^2T_{a,i,c,k} \quad {}^2T_{b,l,d,j} \quad V_{k,d,l,c}$$

Factorized expression

$$\tau^0_{\gamma,\delta,w} = \sum_{a \in V} {}^2D^1_{a,w} Y^1_{a,\gamma} Y^{1,*}_{a,\delta} \quad (3r_D r_T^2 N_v) \quad (13066)$$

$$\tau^1_{\gamma,\alpha} = \sum_{a \in V} W^2_{a,\alpha} Y^3_{a,\gamma} \quad (2r_T r_V N_v) \quad (13067)$$

$$\tau^2_{\gamma,\alpha,i} = \sum_{\beta \in B} W^1_{i,\beta} X_{\beta,\alpha} \tau^1_{\gamma,\beta} \quad (3r_T r_V^2 N_o) \quad (13068)$$

$$\tau^3_{\gamma,\alpha} = \sum_{i \in O} W^3_{i,\alpha} Y^4_{i,\gamma} \quad (2r_T r_V N_o) \quad (13069)$$

$$\tau^4_{\gamma,\alpha} = \sum_{a \in V} W^4_{a,\alpha} Y^3_{a,\gamma} \quad (2r_T r_V N_v) \quad (13070)$$

$$\tau^5_{\gamma,\delta,i} = \sum_{\alpha \in B} \tau^3_{\gamma,\alpha} \tau^4_{\delta,\alpha} \tau^2_{\gamma,\alpha,i} \quad (3r_T^2 r_V N_o) \quad (13071)$$

$$\tau^6_{\gamma,\delta,\epsilon} = \sum_{i \in O} Y^2_{i,\gamma} Z_{\gamma,\delta} \tau^5_{\epsilon,\delta,i} \quad (3r_T^3 N_o) \quad (13072)$$

$$\tau^7_{\gamma,\delta,i} = \sum_{\epsilon \in A} Y^4_{i,\epsilon} \tau^6_{\gamma,\epsilon,\delta} \quad (2r_T^3 N_o) \quad (13073)$$

$$\tau^8_{\gamma,\delta,w} = \sum_{\epsilon \in A} \sum_{i \in O} {}^2D^2_{i,w} Y^{2,*}_{i,\delta} \tau^0_{\epsilon,\delta,w} \tau^7_{\epsilon,\gamma,i} \quad (4r_D r_T^3 N_o) \quad (13074)$$

$$\tau^9_{\gamma,\delta,w} = \sum_{\epsilon \in A} Z^*_{\epsilon,\delta} \tau^8_{\gamma,\epsilon,w} \quad (2r_D r_T^3) \quad (13075)$$

$$\tau^{10}_{\gamma,\delta,w} = \sum_{\epsilon \in A} Z_{\gamma,\epsilon} \tau^9_{\epsilon,\delta,w} \quad (2r_D r_T^3) \quad (13076)$$

$$\tau^{11}_{\gamma,\delta,w} = \sum_{a \in V} {}^2D^3_{a,w} Y^1_{a,\gamma} Y^{3,*}_{a,\delta} \quad (3r_D r_T^2 N_v) \quad (13077)$$

$${}^2R^4_{i,\gamma} \leftarrow \sum_{\delta \in A} \sum_{w \in D} \frac{1}{4} {}^2D^4_{i,w} Y^2_{i,\delta} \tau^{10}_{\delta,\gamma,w} \tau^{11}_{\delta,\gamma,w} \quad (4r_D r_T^2 N_o) \quad (13078)$$

Raw expression

$${}^2R^4_{j,\zeta} \leftarrow \sum_{\gamma \in A} \sum_{i \in O} \sum_{k \in O} \sum_{l \in O} \sum_{a \in V} \sum_{b \in V} \sum_{c \in V} \sum_{d \in V} \frac{1}{4} \quad (13079)$$

$$Y^{1,*}_{a,\gamma} \quad Y^{2,*}_{i,\gamma} \quad Z^*_{\gamma,\zeta} \quad Y^{3,*}_{b,\zeta}$$

$${}^2D^{a,i,b,j} \quad {}^2T_{a,i,c,k} \quad {}^2T_{d,j,b,l} \quad V_{k,d,l,c}$$

Factorized expression

$$\tau^0_{\gamma,\delta,w} = \sum_{a \in V} {}^2D^3_{a,w} Y^1_{a,\gamma} Y^{3,*}_{a,\delta} \quad (3r_D r_T^2 N_v) \quad (13080)$$

$$\tau^1_{\gamma,\alpha} = \sum_{a \in V} W^2_{a,\alpha} Y^3_{a,\gamma} \quad (2r_T r_V N_v) \quad (13081)$$

$$\tau^2_{\gamma,\alpha,i} = \sum_{\beta \in B} W^1_{i,\beta} X_{\beta,\alpha} \tau^1_{\gamma,\beta} \quad (3r_T r_V^2 N_o) \quad (13082)$$

$$\tau^3_{\gamma,\alpha} = \sum_{i \in O} W^3_{i,\alpha} Y^4_{i,\gamma} \quad (2r_T r_V N_o) \quad (13083)$$

$$\tau^4_{\gamma,\alpha} = \sum_{\delta \in A} \sum_{i \in O} Y^2_{i,\gamma} Z_{\gamma,\delta} \tau^3_{\delta,\alpha} \tau^2_{\delta,\alpha,i} \quad (4r_T^2 r_V N_o) \quad (13084)$$

$$\tau^5_{\gamma,a} = \sum_{\alpha \in B} W^4_{a,\alpha} \tau^4_{\gamma,\alpha} \quad (2r_T r_V N_v) \quad (13085)$$

$$\tau^6_{\gamma,\delta} = \sum_{a \in V} Y^3_{a,\delta} \tau^5_{\gamma,a} \quad (2r_T^2 N_v) \quad (13086)$$

$$\tau^7_{\gamma,a} = \sum_{\delta \in A} Y^1_{a,\delta} \tau^6_{\delta,\gamma} \quad (2r_T^2 N_v) \quad (13087)$$

$$\tau^8_{\gamma,\delta,w} = \sum_{a \in V} {}^2D^1_{a,w} Y^{1,*}_{a,\delta} \tau^7_{\gamma,a} \quad (3r_D r_T^2 N_v) \quad (13088)$$

$$\tau^9_{\gamma,\delta,w} = \sum_{i \in O} {}^2D^2_{i,w} Y^4_{i,\gamma} Y^{2,*}_{i,\delta} \quad (3r_D r_T^2 N_o) \quad (13089)$$

$$\tau_{\gamma,\delta,w}^{10} = \sum_{\epsilon \in A} Z_{\epsilon,\delta}^* \tau_{\gamma,\epsilon,w}^8 \tau_{\gamma,\epsilon,w}^9 \quad (3r_D r_T^3) \quad (13090)$$

$$\tau_{\gamma,\alpha,i}^9 = \sum_{\delta \in A} Z_{\gamma,\delta} Y_{i,\delta}^4 \tau_{\delta,\alpha}^8 \quad (3r_T^2 r_V N_o) \quad (13103)$$

$$\tau_{\gamma,\delta,w}^{11} = \sum_{\epsilon \in A} Z_{\gamma,\epsilon} \tau_{\epsilon,\delta,w}^{10} \quad (2r_D r_T^3) \quad (13091)$$

$$\tau_{\gamma,\delta,w,i}^{10} = \sum_{\alpha \in B} \tau_{\gamma,\alpha}^7 \tau_{\delta,\alpha,w}^6 \tau_{\gamma,\alpha,i}^9 \quad (3r_D r_T^2 r_V N_o) \quad (13104)$$

$${}^2R_{i,\gamma}^4 \leftarrow \sum_{\delta \in A} \sum_{w \in D} \frac{1}{4} {}^2D_{i,w}^4 Y_{i,\delta}^2 \tau_{\delta,\gamma,w}^0 \tau_{\delta,\gamma,w}^{11} \quad (4r_D r_T^2 N_o) \quad (13092)$$

$$\tau_{\gamma,\delta,w}^{11} = \sum_{a \in V} {}^2D_{a,w}^3 Y_{a,\gamma}^1 Y_{a,\delta}^{3,*} \quad (3r_D r_T^2 N_v) \quad (13105)$$

Raw expression

$${}^2R_{j,\zeta}^4 \leftarrow \sum_{\gamma \in A} \sum_{i \in O} \sum_{k \in O} \sum_{l \in O} \sum_{a \in V} \sum_{b \in V} \sum_{c \in V} \sum_{d \in V} \frac{1}{4} \quad (13093)$$

$$Y_{a,\gamma}^{1,*} Y_{i,\gamma}^{2,*} Z_{\gamma,\zeta}^* Y_{b,\zeta}^{3,*}$$

$${}^2D_{a,i,b,j} {}^2T_{a,i,d,j} {}^2T_{b,k,c,l} V_{k,c,l,d}$$

$$\tau_{\gamma,w,i}^{12} = \sum_{\delta \in A} \tau_{\delta,\gamma,w}^{11} \tau_{\delta,\gamma,w,i}^{10} \quad (2r_D r_T^2 N_o) \quad (13106)$$

$${}^2R_{i,\gamma}^4 \leftarrow \sum_{w \in D} \frac{1}{4} {}^2D_{i,w}^4 \tau_{\gamma,w,i}^{12} \quad (2r_D r_T N_o) \quad (13107)$$

Factorized expression

$$\tau_{\gamma,\delta,w}^0 = \sum_{a \in V} {}^2D_{a,w}^1 Y_{a,\gamma}^1 Y_{a,\delta}^{1,*} \quad (3r_D r_T^2 N_v) \quad (13094)$$

$${}^2R_{j,\zeta}^4 \leftarrow \sum_{\gamma \in A} \sum_{i \in O} \sum_{k \in O} \sum_{l \in O} \sum_{a \in V} \sum_{b \in V} \sum_{c \in V} \sum_{d \in V} \frac{1}{4} \quad (13108)$$

$$Y_{a,\gamma}^{1,*} Y_{i,\gamma}^{2,*} Z_{\gamma,\zeta}^* Y_{b,\zeta}^{3,*}$$

$${}^2D_{a,i,b,j} {}^2T_{a,i,d,j} {}^2T_{c,k,b,l} V_{k,d,l,c}$$

Raw expression

$$\tau_{\gamma,\alpha}^1 = \sum_{i \in O} W_{i,\alpha}^1 Y_{i,\gamma}^2 \quad (2r_T r_V N_o) \quad (13095)$$

Factorized expression

$$\tau_{\gamma,\alpha}^2 = \sum_{a \in V} W_{a,\alpha}^2 Y_{a,\gamma}^3 \quad (2r_T r_V N_v) \quad (13096)$$

$$\tau_{\gamma,\delta,w}^0 = \sum_{a \in V} {}^2D_{a,w}^1 Y_{a,\gamma}^1 Y_{a,\delta}^{1,*} \quad (3r_D r_T^2 N_v) \quad (13109)$$

$$\tau_{\gamma,\alpha,i}^3 = \sum_{\delta \in A} Z_{\gamma,\delta} Y_{i,\delta}^4 \tau_{\delta,\alpha}^2 \quad (3r_T^2 r_V N_o) \quad (13097)$$

$$\tau_{\gamma,\delta,w}^1 = \sum_{i \in O} {}^2D_{i,w}^2 Y_{i,\gamma}^2 Y_{i,\delta}^{2,*} \quad (3r_D r_T^2 N_o) \quad (13110)$$

$$\tau_{\gamma,\alpha,w}^4 = \sum_{\delta \in A} \sum_{i \in O} {}^2D_{i,w}^2 Y_{i,\gamma}^{2,*} \tau_{\delta,\alpha}^1 \tau_{\delta,\gamma,w}^0 \tau_{\delta,\alpha,i}^3 \quad (5r_D r_T^2 r_V N_o) \quad (13098)$$

$$\tau_{\gamma,\delta,w}^2 = \sum_{\epsilon \in A} Z_{\epsilon,\delta}^* \tau_{\gamma,\epsilon,w}^0 \tau_{\gamma,\epsilon,w}^1 \quad (3r_D r_T^3) \quad (13111)$$

$$\tau_{\gamma,\alpha,w}^5 = \sum_{\beta \in B} X_{\beta,\alpha} \tau_{\gamma,\beta,w}^4 \quad (2r_D r_T r_V^2) \quad (13099)$$

$$\tau_{\gamma,\delta,w}^3 = \sum_{\epsilon \in A} Z_{\epsilon,\gamma} \tau_{\epsilon,\delta,w}^2 \quad (2r_D r_T^3) \quad (13112)$$

$$\tau_{\gamma,\alpha,w}^6 = \sum_{\delta \in A} Z_{\delta,\gamma}^* \tau_{\delta,\alpha,w}^5 \quad (2r_D r_T^2 r_V) \quad (13100)$$

$$\tau_{\gamma,\alpha}^4 = \sum_{a \in V} W_{a,\alpha}^4 Y_{a,\gamma}^3 \quad (2r_T r_V N_v) \quad (13113)$$

$$\tau_{\gamma,\alpha}^7 = \sum_{i \in O} W_{i,\alpha}^3 Y_{i,\gamma}^2 \quad (2r_T r_V N_o) \quad (13101)$$

$$\tau_{\gamma,\alpha,i}^5 = \sum_{\beta \in B} X_{\alpha,\beta} W_{i,\beta}^3 \tau_{\gamma,\beta}^4 \quad (3r_T r_V^2 N_o) \quad (13114)$$

$$\tau_{\gamma,\alpha}^8 = \sum_{a \in V} W_{a,\alpha}^4 Y_{a,\gamma}^3 \quad (2r_T r_V N_v) \quad (13102)$$

$$\tau_{\gamma,\alpha}^6 = \sum_{i \in O} W_{i,\alpha}^1 Y_{i,\gamma}^4 \quad (2r_T r_V N_o) \quad (13115)$$

$$\tau^7_{\gamma,\alpha} = \sum_{a \in V} W^2_{a,\alpha} Y^1_{a,\gamma} \quad (2r_T r_V N_v) \quad (13116)$$

$$\tau^4_{\gamma,\delta,i} = \sum_{\alpha \in B} \tau^2_{\gamma,\alpha} \tau^3_{\delta,\alpha} \tau^1_{\gamma,\alpha,i} \quad (3r_T^2 r_V N_o) \quad (13129)$$

$$\tau^8_{\gamma,\delta,i} = \sum_{\alpha \in B} \tau^6_{\delta,\alpha} \tau^7_{\gamma,\alpha} \tau^5_{\delta,\alpha,i} \quad (3r_T^2 r_V N_o) \quad (13117)$$

$$\tau^5_{\gamma,i} = \sum_{\delta \in A} Z_{\delta,\gamma} \tau^4_{\delta,\gamma,i} \quad (2r_T^2 N_o) \quad (13130)$$

$$\tau^9_{\gamma,\delta,\epsilon} = \sum_{i \in O} Z_{\gamma,\delta} Y^4_{i,\delta} \tau^8_{\gamma,\epsilon,i} \quad (3r_T^3 N_o) \quad (13118)$$

$$\tau^6_{i,j} = \sum_{\gamma \in A} Y^4_{j,\gamma} \tau^5_{\gamma,i} \quad (2r_T N_o^2) \quad (13131)$$

$$\tau^{10}_{\gamma,\delta,i} = \sum_{\epsilon \in A} Y^2_{i,\epsilon} \tau^9_{\epsilon,\gamma,\delta} \quad (2r_T^3 N_o) \quad (13119)$$

$$\tau^7_{\gamma,i} = \sum_{j \in O} Y^4_{j,\gamma} \tau^6_{j,i} \quad (2r_T N_o^2) \quad (13132)$$

$$\tau^{11}_{\gamma,\delta,w,i} = \sum_{\epsilon \in A} \tau^{10}_{\gamma,\epsilon,i} \tau^3_{\epsilon,\delta,w} \quad (2r_D r_T^3 N_o) \quad (13120)$$

$$\tau^8_{\gamma,\delta,w} = \sum_{a \in V} {}^2D^3_{a,w} Y^3_{a,\gamma} Y^{3,*}_{a,\delta} \quad (3r_D r_T^2 N_v) \quad (13133)$$

$$\tau^{12}_{\gamma,\delta,w} = \sum_{a \in V} {}^2D^3_{a,w} Y^3_{a,\gamma} Y^{3,*}_{a,\delta} \quad (3r_D r_T^2 N_v) \quad (13121)$$

$$\tau^9_{\gamma,\delta,w} = \sum_{a \in V} {}^2D^1_{a,w} Y^1_{a,\gamma} Y^{1,*}_{a,\delta} \quad (3r_D r_T^2 N_v) \quad (13134)$$

$$\tau^{13}_{\gamma,w,i} = \sum_{\delta \in A} \tau^{12}_{\delta,\gamma,w} \tau^{11}_{\delta,\gamma,w,i} \quad (2r_D r_T^2 N_o) \quad (13122)$$

$$\tau^{10}_{\gamma,\delta,w} = \sum_{i \in O} {}^2D^2_{i,w} Y^2_{i,\gamma} Y^{2,*}_{i,\delta} \quad (3r_D r_T^2 N_o) \quad (13135)$$

$${}^2R^4_{i,\gamma} \leftarrow \sum_{w \in D} \frac{1}{4} {}^2D^4_{i,w} \tau^{13}_{\gamma,w,i} \quad (2r_D r_T N_o) \quad (13123)$$

$$\tau^{11}_{\gamma,\delta,w} = \sum_{\epsilon \in A} Z^*_{\epsilon,\delta} \tau^{10}_{\gamma,\epsilon,w} \tau^9_{\gamma,\epsilon,w} \quad (3r_D r_T^3) \quad (13136)$$

Raw expression

$${}^2R^4_{j,\zeta} \leftarrow \sum_{\gamma \in A} \sum_{i \in O} \sum_{k \in O} \sum_{l \in O} \sum_{a \in V} \sum_{b \in V} \sum_{c \in V} \sum_{d \in V} \frac{1}{4} \quad (13124)$$

$$Y^{1,*}_{a,\gamma} Y^{2,*}_{i,\gamma} Z^*_{\gamma,\zeta} Y^{3,*}_{b,\zeta}$$

$${}^2D^{a,i,b,j} {}^2T_{a,k,b,l} {}^2T_{c,i,d,j} V_{k,c,l,d}$$

$$\tau^{12}_{\gamma,\delta,w} = \sum_{\epsilon \in A} Z_{\epsilon,\gamma} \tau^{11}_{\epsilon,\delta,w} \quad (2r_D r_T^3) \quad (13137)$$

$${}^2R^4_{i,\gamma} \leftarrow \sum_{\delta \in A} \sum_{w \in D} \frac{1}{4} {}^2D^4_{i,w} \tau^7_{\delta,i} \tau^{12}_{\delta,\gamma,w} \tau^8_{\delta,\gamma,w} \quad (4r_D r_T^2 N_o) \quad (13138)$$

Factorized expression

$$\tau^0_{\gamma,\alpha} = \sum_{a \in V} W^2_{a,\alpha} Y^1_{a,\gamma} \quad (2r_T r_V N_v) \quad (13125)$$

Raw expression

$$\tau^1_{\gamma,\alpha,i} = \sum_{\beta \in B} W^1_{i,\beta} X_{\beta,\alpha} \tau^0_{\gamma,\beta} \quad (3r_T r_V^2 N_o) \quad (13126)$$

$${}^2R^4_{j,\zeta} \leftarrow \sum_{\gamma \in A} \sum_{i \in O} \sum_{k \in O} \sum_{l \in O} \sum_{a \in V} \sum_{b \in V} \sum_{c \in V} \sum_{d \in V} \frac{1}{4} \quad (13139)$$

$$Y^{1,*}_{a,\gamma} Y^{2,*}_{i,\gamma} Z^*_{\gamma,\zeta} Y^{3,*}_{b,\zeta}$$

$${}^2D^{a,i,b,j} {}^2T_{a,k,b,l} {}^2T_{c,j,d,i} V_{k,d,l,c}$$

$$\tau^2_{\gamma,\alpha} = \sum_{i \in O} W^3_{i,\alpha} Y^2_{i,\gamma} \quad (2r_T r_V N_o) \quad (13127)$$

Factorized expression

$$\tau^3_{\gamma,\alpha} = \sum_{a \in V} W^4_{a,\alpha} Y^3_{a,\gamma} \quad (2r_T r_V N_v) \quad (13128)$$

$$\tau^0_{\gamma,\delta,w} = \sum_{a \in V} {}^2D^3_{a,w} Y^3_{a,\gamma} Y^{3,*}_{a,\delta} \quad (3r_D r_T^2 N_v) \quad (13140)$$

$$\tau^1_{\gamma,\delta,w,i} = \sum_{\epsilon \in A} Z_{\gamma,\epsilon} Y^4_{i,\epsilon} \tau^0_{\epsilon,\delta,w} \quad (3r_D r_T^3 N_o) \quad (13141)$$

$$\tau^2_{\gamma,\delta,\alpha,w} = \sum_{i \in O} W^3_{i,\alpha} \tau^1_{\gamma,\delta,w,i} \quad (2r_D r_T^2 r_V N_o) \quad (13142)$$

$$\tau^3_{\gamma,\alpha} = \sum_{a \in V} W^2_{a,\alpha} Y^1_{a,\gamma} \quad (2r_T r_V N_v) \quad (13143)$$

$$\tau^4_{\gamma,\alpha,i} = \sum_{\beta \in B} W^1_{i,\beta} X_{\beta,\alpha} \tau^3_{\gamma,\beta} \quad (3r_T r_V^2 N_o) \quad (13144)$$

$$\tau^5_{\gamma,\delta,\alpha} = \sum_{i \in O} Y^2_{i,\delta} \tau^4_{\gamma,\alpha,i} \quad (2r_T^2 r_V N_o) \quad (13145)$$

$$\tau^6_{\gamma,\delta,w} = \sum_{a \in V} {}^2D^1_{a,w} Y^1_{a,\gamma} Y^{1,*}_{a,\delta} \quad (3r_D r_T^2 N_v) \quad (13146)$$

$$\tau^7_{\gamma,\delta,w,i} = \sum_{\epsilon \in A} Y^{2,*}_{i,\epsilon} Z^*_{\epsilon,\delta} \tau^6_{\gamma,\epsilon,w} \quad (3r_D r_T^3 N_o) \quad (13147)$$

$$\tau^8_{\gamma,\delta,\epsilon,w} = \sum_{i \in O} {}^2D^2_{i,w} Y^2_{i,\delta} \tau^7_{\gamma,\epsilon,w,i} \quad (3r_D r_T^3 N_o) \quad (13148)$$

$$\tau^9_{\gamma,\delta,\alpha,w} = \sum_{\epsilon \in A} \tau^5_{\epsilon,\gamma,\alpha} \tau^2_{\epsilon,\delta,\alpha,w} \tau^8_{\gamma,\epsilon,\delta,w} \quad (3r_D r_T^3 r_V) \quad (13149)$$

$$\tau^{10}_{\gamma,\alpha} = \sum_{a \in V} W^4_{a,\alpha} Y^3_{a,\gamma} \quad (2r_T r_V N_v) \quad (13150)$$

$$\tau^{11}_{\gamma,\alpha,i} = \sum_{\delta \in A} Z_{\gamma,\delta} Y^4_{i,\delta} \tau^{10}_{\delta,\alpha} \quad (3r_T^2 r_V N_o) \quad (13151)$$

$$\tau^{12}_{\gamma,w,i} = \sum_{\delta \in A} \sum_{\alpha \in B} \tau^{11}_{\delta,\alpha,i} \tau^9_{\delta,\gamma,\alpha,w} \quad (2r_D r_T^2 r_V N_o) \quad (13152)$$

$${}^2R^4_{i,\gamma} \leftarrow \sum_{w \in D} \frac{1}{4} {}^2D^4_{i,w} \tau^{12}_{\gamma,w,i} \quad (2r_D r_T N_o) \quad (13153)$$

Raw expression

$${}^2R^4_{j,\zeta} \leftarrow \sum_{\gamma \in A} \sum_{i \in O} \sum_{k \in O} \sum_{l \in O} \sum_{a \in V} \sum_{b \in V} \sum_{c \in V} \sum_{d \in V} \frac{1}{4} \quad (13154)$$

$$Y^{1,*}_{a,\gamma} Y^{2,*}_{i,\gamma} Z^*_{\gamma,\zeta} Y^{3,*}_{b,\zeta}$$

$${}^2D^{a,i,b,j} {}^2T_{a,k,c,i} {}^2T_{b,j,d,l} V_{k,d,l,c}$$

Factorized expression

$$\tau^0_{\gamma,\delta,w} = \sum_{a \in V} {}^2D^3_{a,w} Y^3_{a,\gamma} Y^{3,*}_{a,\delta} \quad (3r_D r_T^2 N_v) \quad (13155)$$

$$\tau^1_{\gamma,\delta,w,i} = \sum_{\epsilon \in A} Z_{\gamma,\epsilon} Y^4_{i,\epsilon} \tau^0_{\epsilon,\delta,w} \quad (3r_D r_T^3 N_o) \quad (13156)$$

$$\tau^2_{\gamma,\delta,w} = \sum_{a \in V} {}^2D^1_{a,w} Y^1_{a,\gamma} Y^{1,*}_{a,\delta} \quad (3r_D r_T^2 N_v) \quad (13157)$$

$$\tau^3_{\gamma,\delta,w,i} = \sum_{\epsilon \in A} Y^{2,*}_{i,\epsilon} Z^*_{\epsilon,\delta} \tau^2_{\gamma,\epsilon,w} \quad (3r_D r_T^3 N_o) \quad (13158)$$

$$\tau^4_{\gamma,\alpha} = \sum_{a \in V} W^2_{a,\alpha} Y^1_{a,\gamma} \quad (2r_T r_V N_v) \quad (13159)$$

$$\tau^5_{\gamma,\alpha,i} = \sum_{\beta \in B} W^1_{i,\beta} X_{\beta,\alpha} \tau^4_{\gamma,\beta} \quad (3r_T r_V^2 N_o) \quad (13160)$$

$$\tau^6_{\gamma,\alpha} = \sum_{a \in V} W^4_{a,\alpha} Y^3_{a,\gamma} \quad (2r_T r_V N_v) \quad (13161)$$

$$\tau^7_{\gamma,\alpha,i} = \sum_{\delta \in A} Z_{\gamma,\delta} Y^4_{i,\delta} \tau^6_{\delta,\alpha} \quad (3r_T^2 r_V N_o) \quad (13162)$$

$$\tau^8_{\gamma,i,j,k} = \sum_{\alpha \in B} W^3_{j,\alpha} \tau^5_{\gamma,\alpha,i} \tau^7_{\gamma,\alpha,k} \quad (3r_T r_V N_o^3) \quad (13163)$$

$$\tau^9_{i,j,k,l} = \sum_{\gamma \in A} Y^2_{k,\gamma} \tau^8_{\gamma,i,j,l} \quad (2r_T N_o^4) \quad (13164)$$

$$\tau^{10}_{\gamma,i,j,k} = \sum_{l \in O} Y^2_{l,\gamma} \tau^9_{l,i,j,k} \quad (2r_T N_o^4) \quad (13165)$$

$$\tau^{11}_{\gamma,w,i,j} = \sum_{\delta \in A} \sum_{k \in O} \tau^1_{\delta,\gamma,w,k} \tau^{10}_{\delta,k,i,j} \tau^3_{\delta,\gamma,w,i} \quad (3r_D r_T^2 N_o^3) \quad (13166)$$

$${}^2R^4_{i,\gamma} \leftarrow \sum_{w \in D} \sum_{j \in O} \frac{1}{4} {}^2D^2_{j,w} {}^2D^4_{i,w} \tau^{11}_{\gamma,w,j,i} \quad (3r_D r_T N_o^2) \quad (13167)$$

Raw expression

$${}^2R^4_{j,\zeta} \leftarrow \sum_{\gamma \in A} \sum_{i \in O} \sum_{k \in O} \sum_{l \in O} \sum_{a \in V} \sum_{b \in V} \sum_{c \in V} \sum_{d \in V} \frac{1}{4} \quad (13168)$$

$$Y^{1,*}_{a,\gamma} \quad Y^{2,*}_{i,\gamma} \quad Z^{*}_{\gamma,\zeta} \quad Y^{3,*}_{b,\zeta}$$

$${}^2D^{a,i,b,j} \quad {}^2T_{a,k,c,i} \quad {}^2T_{b,l,d,j} \quad V_{k,c,l,d}$$

Factorized expression

$$\tau^0_{\gamma,\delta,w} = \sum_{a \in V} {}^2D^1_{a,w} Y^1_{a,\gamma} Y^{1,*}_{a,\delta} \quad (3r_D r_T^2 N_v) \quad (13169)$$

$$\tau^1_{\gamma,\alpha} = \sum_{a \in V} W^2_{a,\alpha} Y^1_{a,\gamma} \quad (2r_T r_V N_v) \quad (13170)$$

$$\tau^2_{\gamma,\alpha,i} = \sum_{\beta \in B} W^1_{i,\beta} X_{\beta,\alpha} \tau^1_{\gamma,\beta} \quad (3r_T r_V^2 N_o) \quad (13171)$$

$$\tau^3_{\gamma,\alpha} = \sum_{i \in O} W^3_{i,\alpha} Y^2_{i,\gamma} \quad (2r_T r_V N_o) \quad (13172)$$

$$\tau^4_{\gamma,\alpha} = \sum_{a \in V} W^4_{a,\alpha} Y^3_{a,\gamma} \quad (2r_T r_V N_v) \quad (13173)$$

$$\tau^5_{\gamma,\delta,i} = \sum_{\alpha \in B} \tau^3_{\gamma,\alpha} \tau^4_{\delta,\alpha} \tau^2_{\gamma,\alpha,i} \quad (3r_T^2 r_V N_o) \quad (13174)$$

$$\tau^6_{\gamma,\delta,\epsilon} = \sum_{i \in O} Y^2_{i,\delta} Z_{\delta,\epsilon} \tau^5_{\gamma,\epsilon,i} \quad (3r_T^3 N_o) \quad (13175)$$

$$\tau^7_{\gamma,\delta,i} = \sum_{\epsilon \in A} Y^4_{i,\epsilon} \tau^6_{\gamma,\delta,\epsilon} \quad (2r_T^3 N_o) \quad (13176)$$

$$\tau^8_{\gamma,\delta,w} = \sum_{\epsilon \in A} \sum_{i \in O} {}^2D^2_{i,w} Y^{2,*}_{i,\delta} \tau^0_{\epsilon,\delta,w} \tau^7_{\gamma,\epsilon,i} \quad (4r_D r_T^3 N_o) \quad (13177)$$

$$\tau^9_{\gamma,\delta,w} = \sum_{\epsilon \in A} Z^{*}_{\epsilon,\delta} \tau^8_{\gamma,\epsilon,w} \quad (2r_D r_T^3) \quad (13178)$$

$$\tau^{10}_{\gamma,\delta,w} = \sum_{\epsilon \in A} Z_{\epsilon,\gamma} \tau^9_{\epsilon,\delta,w} \quad (2r_D r_T^3) \quad (13179)$$

$$\tau^{11}_{\gamma,\delta,w} = \sum_{a \in V} {}^2D^3_{a,w} Y^3_{a,\gamma} Y^{3,*}_{a,\delta} \quad (3r_D r_T^2 N_v) \quad (13180)$$

$${}^2R^4_{i,\gamma} \leftarrow \sum_{\delta \in A} \sum_{w \in D} \frac{1}{4} {}^2D^4_{i,w} Y^4_{i,\delta} \tau^{10}_{\delta,\gamma,w} \tau^{11}_{\delta,\gamma,w} \quad (4r_D r_T^2 N_o) \quad (13181)$$

Raw expression

$${}^2R^4_{j,\zeta} \leftarrow \sum_{\gamma \in A} \sum_{i \in O} \sum_{k \in O} \sum_{l \in O} \sum_{a \in V} \sum_{b \in V} \sum_{c \in V} \sum_{d \in V} \frac{1}{4} \quad (13182)$$

$$Y^{1,*}_{a,\gamma} \quad Y^{2,*}_{i,\gamma} \quad Z^{*}_{\gamma,\zeta} \quad Y^{3,*}_{b,\zeta}$$

$${}^2D^{a,i,b,j} \quad {}^2T_{a,k,c,i} \quad {}^2T_{d,j,b,l} \quad V_{k,c,l,d}$$

Factorized expression

$$\tau^0_{\gamma,\alpha} = \sum_{a \in V} W^2_{a,\alpha} Y^3_{a,\gamma} \quad (2r_T r_V N_v) \quad (13183)$$

$$\tau^1_{\gamma,\alpha,i} = \sum_{\beta \in B} W^1_{i,\beta} X_{\beta,\alpha} \tau^0_{\gamma,\beta} \quad (3r_T r_V^2 N_o) \quad (13184)$$

$$\tau^2_{\gamma,\alpha} = \sum_{i \in O} W^3_{i,\alpha} Y^4_{i,\gamma} \quad (2r_T r_V N_o) \quad (13185)$$

$$\tau^3_{\gamma,\alpha} = \sum_{a \in V} W^4_{a,\alpha} Y^1_{a,\gamma} \quad (2r_T r_V N_v) \quad (13186)$$

$$\tau^4_{\gamma,\delta,i} = \sum_{\alpha \in B} \tau^2_{\delta,\alpha} \tau^3_{\gamma,\alpha} \tau^1_{\delta,\alpha,i} \quad (3r_T^2 r_V N_o) \quad (13187)$$

$$\tau^5_{\gamma,i} = \sum_{\delta \in A} Z_{\gamma,\delta} \tau^4_{\gamma,\delta,i} \quad (2r_T^2 N_o) \quad (13188)$$

$$\tau^6_{i,j} = \sum_{\gamma \in A} Y^2_{j,\gamma} \tau^5_{\gamma,i} \quad (2r_T N_o^2) \quad (13189)$$

$$\tau^7_{\gamma,i} = \sum_{j \in O} Y^4_{j,\gamma} \tau^6_{j,i} \quad (2r_T N_o^2) \quad (13190)$$

$$\tau^8_{\gamma,\delta,w} = \sum_{a \in V} {}^2D^3_{a,w} Y^3_{a,\gamma} Y^{3,*}_{a,\delta} \quad (3r_D r_T^2 N_v) \quad (13191)$$



$$\tau_{\gamma,\delta,w}^9 = \sum_{a \in V} {}^2D_{a,w}^1 Y_{a,\gamma}^1 Y_{a,\delta}^{1,*} \quad (3r_D r_T^2 N_v) \quad (13192)$$

$$\tau_{\gamma,\alpha}^6 = \sum_{i \in O} W_{i,\alpha}^1 Y_{i,\gamma}^2 \quad (2r_T r_V N_o) \quad (13204)$$

$$\tau_{\gamma,\delta,w}^{10} = \sum_{i \in O} {}^2D_{i,w}^2 Y_{i,\gamma}^2 Y_{i,\delta}^{2,*} \quad (3r_D r_T^2 N_o) \quad (13193)$$

$$\tau_{\gamma,\alpha}^7 = \sum_{\delta \in A} \sum_{i \in O} Z_{\delta,\gamma} Y_{i,\gamma}^4 \tau_{\delta,\alpha}^6 \tau_{\delta,\alpha,i}^5 \quad (4r_T^2 r_V N_o) \quad (13205)$$

$$\tau_{\gamma,\delta,w}^{11} = \sum_{\epsilon \in A} Z_{\epsilon,\delta}^* \tau_{\gamma,\epsilon,w}^{10} \tau_{\gamma,\epsilon,w}^9 \quad (3r_D r_T^3) \quad (13194)$$

$$\tau_{\gamma,a}^8 = \sum_{\alpha \in B} W_{a,\alpha}^2 \tau_{\gamma,\alpha}^7 \quad (2r_T r_V N_v) \quad (13206)$$

$$\tau_{\gamma,\delta,w}^{12} = \sum_{\epsilon \in A} Z_{\epsilon,\gamma} \tau_{\epsilon,\delta,w}^{11} \quad (2r_D r_T^3) \quad (13195)$$

$$\tau_{a,b}^9 = \sum_{\gamma \in A} Y_{b,\gamma}^3 \tau_{\gamma,a}^8 \quad (2r_T N_v^2) \quad (13207)$$

$${}^2R_{i,\gamma}^4 \leftarrow \sum_{\delta \in A} \sum_{w \in D} \frac{1}{4} {}^2D_{i,w}^4 \tau_{\delta,i}^7 \tau_{\delta,\gamma,w}^{12} \tau_{\delta,\gamma,w}^8 \quad (4r_D r_T^2 N_o) \quad (13196)$$

$$\tau_{\gamma,a}^{10} = \sum_{b \in V} Y_{b,\gamma}^3 \tau_{b,a}^9 \quad (2r_T N_v^2) \quad (13208)$$

$$\tau_{\gamma,\delta,w}^{11} = \sum_{a \in V} {}^2D_{a,w}^3 Y_{a,\delta}^{3,*} \tau_{\gamma,a}^{10} \quad (3r_D r_T^2 N_v) \quad (13209)$$

Raw expression

$${}^2R_{j,\zeta}^4 \leftarrow \sum_{\gamma \in A} \sum_{i \in O} \sum_{k \in O} \sum_{l \in O} \sum_{a \in V} \sum_{b \in V} \sum_{c \in V} \sum_{d \in V} \frac{1}{4} \quad (13197)$$

$$Y_{a,\gamma}^{1,*} Y_{i,\gamma}^{2,*} Z_{\gamma,\zeta}^* Y_{b,\zeta}^{3,*} {}^2D_{a,i,b,j} {}^2T_{a,k,c,i} {}^2T_{d,l,b,j} V_{k,d,l,c}$$

$${}^2R_{i,\gamma}^4 \leftarrow \sum_{\delta \in A} \sum_{w \in D} \frac{1}{4} {}^2D_{i,w}^4 Y_{i,\delta}^4 \tau_{\delta,\gamma,w}^{11} \tau_{\delta,\gamma,w}^3 \quad (4r_D r_T^2 N_o) \quad (13210)$$

Factorized expression

Raw expression

$$\tau_{\gamma,\delta,w}^0 = \sum_{a \in V} {}^2D_{a,w}^1 Y_{a,\gamma}^1 Y_{a,\delta}^{1,*} \quad (3r_D r_T^2 N_v) \quad (13198)$$

$${}^2R_{j,\zeta}^4 \leftarrow \sum_{\gamma \in A} \sum_{i \in O} \sum_{k \in O} \sum_{l \in O} \sum_{a \in V} \sum_{b \in V} \sum_{c \in V} \sum_{d \in V} \frac{1}{4} \quad (13211)$$

$$Y_{a,\gamma}^{1,*} Y_{i,\gamma}^{2,*} Z_{\gamma,\zeta}^* Y_{b,\zeta}^{3,*} {}^2D_{a,i,b,j} {}^2T_{a,k,c,l} {}^2T_{b,j,d,i} V_{k,c,l,d}$$

$$\tau_{\gamma,\delta,w}^1 = \sum_{i \in O} {}^2D_{i,w}^2 Y_{i,\gamma}^2 Y_{i,\delta}^{2,*} \quad (3r_D r_T^2 N_o) \quad (13199)$$

Factorized expression

$$\tau_{\gamma,\delta,w}^2 = \sum_{\epsilon \in A} Z_{\epsilon,\delta}^* \tau_{\gamma,\epsilon,w}^0 \tau_{\gamma,\epsilon,w}^1 \quad (3r_D r_T^3) \quad (13200)$$

$$\tau_{\gamma,\delta,w}^0 = \sum_{a \in V} {}^2D_{a,w}^3 Y_{a,\gamma}^3 Y_{a,\delta}^{3,*} \quad (3r_D r_T^2 N_v) \quad (13212)$$

$$\tau_{\gamma,\delta,w}^3 = \sum_{\epsilon \in A} Z_{\epsilon,\gamma} \tau_{\epsilon,\delta,w}^2 \quad (2r_D r_T^3) \quad (13201)$$

$$\tau_{\gamma,\alpha}^1 = \sum_{a \in V} W_{a,\alpha}^2 Y_{a,\gamma}^3 \quad (2r_T r_V N_v) \quad (13213)$$

$$\tau_{\gamma,\alpha}^4 = \sum_{a \in V} W_{a,\alpha}^4 Y_{a,\gamma}^1 \quad (2r_T r_V N_v) \quad (13202)$$

$$\tau_{\gamma,\alpha,i}^2 = \sum_{\beta \in B} W_{i,\beta}^1 X_{\beta,\alpha} \tau_{\gamma,\beta}^1 \quad (3r_T r_V^2 N_o) \quad (13214)$$

$$\tau_{\gamma,\alpha,i}^5 = \sum_{\beta \in B} X_{\alpha,\beta} W_{i,\beta}^3 \tau_{\gamma,\beta}^4 \quad (3r_T r_V^2 N_o) \quad (13203)$$

$$\tau_{\gamma,\alpha}^3 = \sum_{i \in O} W_{i,\alpha}^3 Y_{i,\gamma}^4 \quad (2r_T r_V N_o) \quad (13215)$$

$$\tau^4_{\gamma,\alpha} = \sum_{a \in V} W^4_{a,\alpha} Y^1_{a,\gamma} \quad (2r_T r_V N_v) \quad (13216)$$

$$\tau^2_{\gamma,\alpha} = \sum_{a \in V} W^2_{a,\alpha} Y^3_{a,\gamma} \quad (2r_T r_V N_v) \quad (13229)$$

$$\tau^5_{\gamma,\delta,i} = \sum_{\alpha \in B} \tau^3_{\delta,\alpha} \tau^4_{\gamma,\alpha} \tau^2_{\delta,\alpha,i} \quad (3r_T^2 r_V N_o) \quad (13217)$$

$$\tau^3_{\gamma,\alpha,i} = \sum_{\beta \in B} W^1_{i,\beta} X_{\beta,\alpha} \tau^2_{\gamma,\beta} \quad (3r_T r_V^2 N_o) \quad (13230)$$

$$\tau^6_{\gamma,i} = \sum_{\delta \in A} Z_{\gamma,\delta} \tau^5_{\gamma,\delta,i} \quad (2r_T^2 N_o) \quad (13218)$$

$$\tau^4_{\gamma,\alpha} = \sum_{i \in O} W^3_{i,\alpha} Y^4_{i,\gamma} \quad (2r_T r_V N_o) \quad (13231)$$

$$\tau^7_{i,j} = \sum_{\gamma \in A} Y^2_{j,\gamma} \tau^6_{\gamma,i} \quad (2r_T N_o^2) \quad (13219)$$

$$\tau^5_{\gamma,\alpha} = \sum_{\delta \in A} \sum_{i \in O} Y^2_{i,\gamma} Z_{\gamma,\delta} \tau^4_{\delta,\alpha} \tau^3_{\delta,\alpha,i} \quad (4r_T^2 r_V N_o) \quad (13232)$$

$$\tau^8_{\gamma,i} = \sum_{j \in O} Y^2_{j,\gamma} \tau^7_{j,i} \quad (2r_T N_o^2) \quad (13220)$$

$$\tau^6_{\gamma,a} = \sum_{\alpha \in B} W^4_{a,\alpha} \tau^5_{\gamma,\alpha} \quad (2r_T r_V N_v) \quad (13233)$$

$$\tau^9_{\gamma,\delta,w} = \sum_{i \in O} {}^2D^2_{i,w} Y^{2,*}_{i,\delta} \tau^8_{\gamma,i} \quad (3r_D r_T^2 N_o) \quad (13221)$$

$$\tau^7_{\gamma,\delta} = \sum_{a \in V} Y^1_{a,\gamma} \tau^6_{\delta,a} \quad (2r_T^2 N_v) \quad (13234)$$

$$\tau^{10}_{\gamma,\delta,w} = \sum_{a \in V} {}^2D^1_{a,w} Y^1_{a,\gamma} Y^{1,*}_{a,\delta} \quad (3r_D r_T^2 N_v) \quad (13222)$$

$$\tau^8_{\gamma,a} = \sum_{\delta \in A} Y^1_{a,\delta} \tau^7_{\gamma,\delta} \quad (2r_T^2 N_v) \quad (13235)$$

$$\tau^{11}_{\gamma,\delta,w} = \sum_{\epsilon \in A} Z^*_{\epsilon,\delta} \tau^{10}_{\gamma,\epsilon,w} \tau^9_{\gamma,\epsilon,w} \quad (3r_D r_T^3) \quad (13223)$$

$$\tau^9_{\gamma,\delta,w} = \sum_{a \in V} {}^2D^1_{a,w} Y^{1,*}_{a,\delta} \tau^8_{\gamma,a} \quad (3r_D r_T^2 N_v) \quad (13236)$$

$$\tau^{12}_{\gamma,\delta,w} = \sum_{\epsilon \in A} Z_{\epsilon,\gamma} \tau^{11}_{\epsilon,\delta,w} \quad (2r_D r_T^3) \quad (13224)$$

$${}^2R^4_{i,\gamma} \leftarrow \sum_{\delta \in A} \sum_{w \in D} \frac{1}{4} {}^2D^4_{i,w} Y^4_{i,\delta} \tau^0_{\delta,\gamma,w} \tau^{12}_{\delta,\gamma,w} \quad (4r_D r_T^2 N_o) \quad (13225)$$

$$\tau^{10}_{\gamma,\delta,w} = \sum_{\epsilon \in A} Z^*_{\epsilon,\delta} \tau^1_{\gamma,\epsilon,w} \tau^9_{\gamma,\epsilon,w} \quad (3r_D r_T^3) \quad (13237)$$

Raw expression

$$\tau^{11}_{\gamma,\delta,w} = \sum_{\epsilon \in A} Z_{\epsilon,\gamma} \tau^{10}_{\epsilon,\delta,w} \quad (2r_D r_T^3) \quad (13238)$$

$${}^2R^4_{j,\zeta} \leftarrow \sum_{\gamma \in A} \sum_{i \in O} \sum_{k \in O} \sum_{l \in O} \sum_{a \in V} \sum_{b \in V} \sum_{c \in V} \sum_{d \in V} \frac{1}{4} Y^{1,*}_{a,\gamma} Y^{2,*}_{i,\gamma} Z^*_{\gamma,\zeta} Y^{3,*}_{b,\zeta} {}^2D^{a,i,b,j}_{a,k,c,l} {}^2T_{a,k,c,l} {}^2T_{d,i,b,j} V_{k,c,l,d} \quad (13226)$$

$${}^2R^4_{i,\gamma} \leftarrow \sum_{\delta \in A} \sum_{w \in D} \frac{1}{4} {}^2D^4_{i,w} Y^4_{i,\delta} \tau^0_{\delta,\gamma,w} \tau^{11}_{\delta,\gamma,w} \quad (4r_D r_T^2 N_o) \quad (13239)$$

Factorized expression

Raw expression

$$\tau^0_{\gamma,\delta,w} = \sum_{a \in V} {}^2D^3_{a,w} Y^3_{a,\gamma} Y^{3,*}_{a,\delta} \quad (3r_D r_T^2 N_v) \quad (13227)$$

$${}^2R^4_{j,\zeta} \leftarrow \sum_{\gamma \in A} \sum_{i \in O} \sum_{k \in O} \sum_{l \in O} \sum_{a \in V} \sum_{b \in V} \sum_{c \in V} \sum_{d \in V} \frac{1}{4} Y^{1,*}_{a,\gamma} Y^{2,*}_{i,\gamma} Z^*_{\gamma,\zeta} Y^{3,*}_{b,\zeta} {}^2D^{a,i,b,j}_{a,k,c,l} {}^2T_{a,k,c,l} {}^2T_{c,i,d,k} V_{l,d,k,c} \quad (13240)$$

$$\tau^1_{\gamma,\delta,w} = \sum_{i \in O} {}^2D^2_{i,w} Y^2_{i,\gamma} Y^{2,*}_{i,\delta} \quad (3r_D r_T^2 N_o) \quad (13228)$$

Factorized expression

Raw expression

$$\tau^0_{\gamma,\delta,w} = \sum_{a \in V} {}^2D^1_{a,w} Y^1_{a,\gamma} Y^{1,*}_{a,\delta} \quad (3r_D r_T^2 N_v) \quad (13241)$$

$$\tau^1_{\gamma,\alpha} = \sum_{i \in O} W^1_{i,\alpha} Y^2_{i,\gamma} \quad (2r_T r_V N_o) \quad (13242)$$

$$\tau^2_{\gamma,\alpha} = \sum_{a \in V} W^2_{a,\alpha} Y^3_{a,\gamma} \quad (2r_T r_V N_v) \quad (13243)$$

$$\tau^3_{\gamma,\alpha,i} = \sum_{\delta \in A} Z_{\gamma,\delta} Y^4_{i,\delta} \tau^2_{\delta,\alpha} \quad (3r_T^2 r_V N_o) \quad (13244)$$

$$\tau^4_{\gamma,\alpha,w} = \sum_{\delta \in A} \sum_{i \in O} {}^2D^2_{i,w} Y^{2,*}_{i,\gamma} \tau^1_{\delta,\alpha} \tau^0_{\delta,\gamma,w} \tau^3_{\delta,\alpha,i} \quad (5r_D r_T^2 r_V N_o) \quad (13245)$$

$$\tau^5_{\gamma,\alpha,w} = \sum_{\beta \in B} X_{\beta,\alpha} \tau^4_{\gamma,\beta,w} \quad (2r_D r_T r_V^2) \quad (13246)$$

$$\tau^6_{\gamma,\alpha,w} = \sum_{\delta \in A} Z^*_{\delta,\gamma} \tau^5_{\delta,\alpha,w} \quad (2r_D r_T^2 r_V) \quad (13247)$$

$$\tau^7_{\gamma,\alpha} = \sum_{a \in V} W^4_{a,\alpha} Y^1_{a,\gamma} \quad (2r_T r_V N_v) \quad (13248)$$

$$\tau^8_{\gamma,\alpha,i} = \sum_{\delta \in A} Y^2_{i,\delta} Z_{\delta,\gamma} \tau^7_{\delta,\alpha} \quad (3r_T^2 r_V N_o) \quad (13249)$$

$$\tau^9_{\gamma,\alpha} = \sum_{i \in O} W^3_{i,\alpha} Y^4_{i,\gamma} \quad (2r_T r_V N_o) \quad (13250)$$

$$\tau^{10}_{\gamma,\delta,w,i} = \sum_{\alpha \in B} \tau^9_{\gamma,\alpha} \tau^6_{\delta,\alpha,w} \tau^8_{\gamma,\alpha,i} \quad (3r_D r_T^2 r_V N_o) \quad (13251)$$

$$\tau^{11}_{\gamma,\delta,w} = \sum_{a \in V} {}^2D^3_{a,w} Y^3_{a,\gamma} Y^{3,*}_{a,\delta} \quad (3r_D r_T^2 N_v) \quad (13252)$$

$$\tau^{12}_{\gamma,w,i} = \sum_{\delta \in A} \tau^{11}_{\delta,\gamma,w} \tau^{10}_{\delta,\gamma,w,i} \quad (2r_D r_T^2 N_o) \quad (13253)$$

$${}^2R^4_{i,\gamma} \leftarrow \sum_{w \in D} \frac{1}{4} {}^2D^4_{i,w} \tau^{12}_{\gamma,w,i} \quad (2r_D r_T N_o) \quad (13254)$$

$${}^2R^4_{j,\zeta} \leftarrow \sum_{\gamma \in A} \sum_{i \in O} \sum_{k \in O} \sum_{l \in O} \sum_{a \in V} \sum_{b \in V} \sum_{c \in V} \sum_{d \in V} \frac{1}{4} \quad (13255)$$

$$Y^{1,*}_{a,\gamma} Y^{2,*}_{i,\gamma} Z^*_{\gamma,\zeta} Y^{3,*}_{b,\zeta} {}^2D^{a,i,b,j} {}^2T_{a,l,b,j} {}^2T_{c,k,d,i} V_{l,c,k,d}$$

Factorized expression

$$\tau^0_{\gamma,\alpha} = \sum_{a \in V} W^4_{a,\alpha} Y^1_{a,\gamma} \quad (2r_T r_V N_v) \quad (13256)$$

$$\tau^1_{\gamma,\alpha,i} = \sum_{\beta \in B} X_{\alpha,\beta} W^3_{i,\beta} \tau^0_{\gamma,\beta} \quad (3r_T r_V^2 N_o) \quad (13257)$$

$$\tau^2_{\gamma,\alpha} = \sum_{a \in V} W^2_{a,\alpha} Y^3_{a,\gamma} \quad (2r_T r_V N_v) \quad (13258)$$

$$\tau^3_{\gamma,\alpha,i} = \sum_{\delta \in A} Z_{\gamma,\delta} Y^4_{i,\delta} \tau^2_{\delta,\alpha} \quad (3r_T^2 r_V N_o) \quad (13259)$$

$$\tau^4_{\gamma,i,j,k} = \sum_{\alpha \in B} W^1_{i,\alpha} \tau^1_{\gamma,\alpha,j} \tau^3_{\gamma,\alpha,k} \quad (3r_T r_V N_o^3) \quad (13260)$$

$$\tau^5_{i,j,k,l} = \sum_{\gamma \in A} Y^{2,k,\gamma} \tau^4_{\gamma,i,j,l} \quad (2r_T N_o^4) \quad (13261)$$

$$\tau^6_{\gamma,i,j,k} = \sum_{l \in O} Y^{2,l,\gamma} \tau^5_{l,i,j,k} \quad (2r_T N_o^4) \quad (13262)$$

$$\tau^7_{\gamma,\delta,w} = \sum_{a \in V} {}^2D^3_{a,w} Y^3_{a,\gamma} Y^{3,*}_{a,\delta} \quad (3r_D r_T^2 N_v) \quad (13263)$$

$$\tau^8_{\gamma,\delta,w,i} = \sum_{\epsilon \in A} Z_{\gamma,\epsilon} Y^4_{i,\epsilon} \tau^7_{\epsilon,\delta,w} \quad (3r_D r_T^3 N_o) \quad (13264)$$

$$\tau^9_{\gamma,\delta,w} = \sum_{a \in V} {}^2D^1_{a,w} Y^1_{a,\gamma} Y^{1,*}_{a,\delta} \quad (3r_D r_T^2 N_v) \quad (13265)$$

$$\tau^{10}_{\gamma,\delta,w,i} = \sum_{\epsilon \in A} Y^{2,*}_{i,\epsilon} Z^*_{\epsilon,\delta} \tau^9_{\gamma,\epsilon,w} \quad (3r_D r_T^3 N_o) \quad (13266)$$

$$\tau^{11}_{\gamma,w,i,j} = \sum_{\delta \in A} \sum_{k \in O} \tau^{10}_{\delta,\gamma,w,j} \tau^6_{\delta,k,i,j} \tau^8_{\delta,\gamma,w,k} \quad (3r_D r_T^2 N_o^3) \quad (13267)$$

$$\tau^9_{\gamma,\delta,\alpha,w} = \sum_{\epsilon \in A} \tau^2_{\gamma,\epsilon,\alpha} \tau^5_{\epsilon,\delta,\alpha,w} \tau^8_{\gamma,\epsilon,\delta,w} \quad (3r_D r_T^3 r_V) \quad (13279)$$

$${}^2R^4_{i,\gamma} \leftarrow \sum_{w \in D} \sum_{j \in O} \frac{1}{4} {}^2D^2_{j,w} {}^2D^4_{i,w} \tau^{11}_{\gamma,w,i,j} \quad (3r_D r_T N_o^2) \quad (13268)$$

$$\tau^{10}_{\gamma,\alpha} = \sum_{a \in V} W^4_{a,\alpha} Y^3_{a,\gamma} \quad (2r_T r_V N_v) \quad (13280)$$

Raw expression

$$\tau^{11}_{\gamma,\alpha,i} = \sum_{\delta \in A} Z_{\gamma,\delta} Y^4_{i,\delta} \tau^{10}_{\delta,\alpha} \quad (3r_T^2 r_V N_o) \quad (13281)$$

$${}^2R^4_{j,\zeta} \leftarrow \sum_{\gamma \in A} \sum_{i \in O} \sum_{k \in O} \sum_{l \in O} \sum_{a \in V} \sum_{b \in V} \sum_{c \in V} \sum_{d \in V} \frac{1}{4} \quad (13269)$$

$$Y^{1,*}_{a,\gamma} Y^{2,*}_{i,\gamma} Z^*_{\gamma,\zeta} Y^{3,*}_{b,\zeta}$$

$${}^2D^{a,i,b,j} {}^2T_{a,l,d,j} {}^2T_{b,k,c,i} V_{l,c,k,d}$$

$$\tau^{12}_{\gamma,w,i} = \sum_{\delta \in A} \sum_{\alpha \in B} \tau^{11}_{\delta,\alpha,i} \tau^9_{\delta,\gamma,\alpha,w} \quad (2r_D r_T^2 r_V N_o) \quad (13282)$$

Factorized expression

$${}^2R^4_{i,\gamma} \leftarrow \sum_{w \in D} \frac{1}{4} {}^2D^4_{i,w} \tau^{12}_{\gamma,w,i} \quad (2r_D r_T N_o) \quad (13283)$$

$$\tau^0_{\gamma,\alpha} = \sum_{a \in V} W^2_{a,\alpha} Y^3_{a,\gamma} \quad (2r_T r_V N_v) \quad (13270)$$

Raw expression

$$\tau^1_{\gamma,\alpha,i} = \sum_{\beta \in B} W^1_{i,\beta} X_{\beta,\alpha} \tau^0_{\gamma,\beta} \quad (3r_T r_V^2 N_o) \quad (13271)$$

$${}^2R^4_{j,\zeta} \leftarrow \sum_{\gamma \in A} \sum_{i \in O} \sum_{k \in O} \sum_{l \in O} \sum_{a \in V} \sum_{b \in V} \sum_{c \in V} \sum_{d \in V} \frac{1}{4} \quad (13284)$$

$$Y^{1,*}_{a,\gamma} Y^{2,*}_{i,\gamma} Z^*_{\gamma,\zeta} Y^{3,*}_{b,\zeta}$$

$${}^2D^{a,i,b,j} {}^2T_{a,l,d,j} {}^2T_{c,i,b,k} V_{l,c,k,d}$$

$$\tau^2_{\gamma,\delta,\alpha} = \sum_{i \in O} Y^2_{i,\gamma} \tau^1_{\delta,\alpha,i} \quad (2r_T^2 r_V N_o) \quad (13272)$$

Factorized expression

$$\tau^3_{\gamma,\delta,w} = \sum_{a \in V} {}^2D^3_{a,w} Y^1_{a,\gamma} Y^{3,*}_{a,\delta} \quad (3r_D r_T^2 N_v) \quad (13273)$$

$$\tau^0_{\gamma,\delta,w} = \sum_{a \in V} {}^2D^3_{a,w} Y^3_{a,\gamma} Y^{3,*}_{a,\delta} \quad (3r_D r_T^2 N_v) \quad (13285)$$

$$\tau^4_{\gamma,\delta,w,i} = \sum_{\epsilon \in A} Y^2_{i,\epsilon} Z_{\epsilon,\gamma} \tau^3_{\epsilon,\delta,w} \quad (3r_D r_T^3 N_o) \quad (13274)$$

$$\tau^1_{\gamma,\alpha} = \sum_{a \in V} W^2_{a,\alpha} Y^1_{a,\gamma} \quad (2r_T r_V N_v) \quad (13286)$$

$$\tau^5_{\gamma,\delta,\alpha,w} = \sum_{i \in O} W^3_{i,\alpha} \tau^4_{\gamma,\delta,w,i} \quad (2r_D r_T^2 r_V N_o) \quad (13275)$$

$$\tau^2_{\gamma,\alpha,i} = \sum_{\beta \in B} W^1_{i,\beta} X_{\beta,\alpha} \tau^1_{\gamma,\beta} \quad (3r_T r_V^2 N_o) \quad (13287)$$

$$\tau^6_{\gamma,\delta,w} = \sum_{a \in V} {}^2D^1_{a,w} Y^1_{a,\gamma} Y^{1,*}_{a,\delta} \quad (3r_D r_T^2 N_v) \quad (13276)$$

$$\tau^3_{\gamma,\alpha} = \sum_{i \in O} W^3_{i,\alpha} Y^2_{i,\gamma} \quad (2r_T r_V N_o) \quad (13288)$$

$$\tau^7_{\gamma,\delta,w,i} = \sum_{\epsilon \in A} Y^{2,*}_{i,\epsilon} Z^*_{\epsilon,\delta} \tau^6_{\gamma,\epsilon,w} \quad (3r_D r_T^3 N_o) \quad (13277)$$

$$\tau^4_{\gamma,\alpha} = \sum_{a \in V} W^4_{a,\alpha} Y^3_{a,\gamma} \quad (2r_T r_V N_v) \quad (13289)$$

$$\tau^5_{\gamma,\delta,i} = \sum_{\alpha \in B} \tau^3_{\gamma,\alpha} \tau^4_{\delta,\alpha} \tau^2_{\gamma,\alpha,i} \quad (3r_T^2 r_V N_o) \quad (13290)$$

$$\tau^8_{\gamma,\delta,\epsilon,w} = \sum_{i \in O} {}^2D^2_{i,w} Y^4_{i,\delta} \tau^7_{\gamma,\epsilon,w,i} \quad (3r_D r_T^3 N_o) \quad (13278)$$

$$\tau^6_{\gamma,i} = \sum_{\delta \in A} Z_{\delta,\gamma} \tau^5_{\delta,\gamma,i} \quad (2r_T^2 N_o) \quad (13291)$$

$$\tau_{i,j}^7 = \sum_{\gamma \in A} Y_{j,\gamma}^4 \tau_{\gamma,i}^6 \quad (2r_T N_o^2) \quad (13292)$$

$$\tau_{\gamma,\alpha}^4 = \sum_{i \in O} W_{i,\alpha}^1 Y_{i,\gamma}^4 \quad (2r_T r_V N_o) \quad (13304)$$

$$\tau_{\gamma,i}^8 = \sum_{j \in O} Y_{j,\gamma}^2 \tau_{j,i}^7 \quad (2r_T N_o^2) \quad (13293)$$

$$\tau_{\gamma,\alpha,w}^5 = \sum_{\delta \in A} \sum_{i \in O} {}^2D_{i,w}^2 Y_{i,\gamma}^{2,*} \tau_{\delta,\alpha}^4 \tau_{\delta,\gamma,w}^1 \tau_{\delta,\alpha,i}^3 \quad (5r_D r_T^2 r_V N_o) \quad (13305)$$

$$\tau_{\gamma,\delta,w}^9 = \sum_{i \in O} {}^2D_{i,w}^2 Y_{i,\delta}^{2,*} \tau_{\gamma,i}^8 \quad (3r_D r_T^2 N_o) \quad (13294)$$

$$\tau_{\gamma,\alpha,w}^6 = \sum_{\beta \in B} X_{\beta,\alpha} \tau_{\gamma,\beta,w}^5 \quad (2r_D r_T r_V^2) \quad (13306)$$

$$\tau_{\gamma,\delta,w}^{10} = \sum_{a \in V} {}^2D_{a,w}^1 Y_{a,\gamma}^1 Y_{a,\delta}^{1,*} \quad (3r_D r_T^2 N_v) \quad (13295)$$

$$\tau_{\gamma,\alpha,w}^7 = \sum_{\delta \in A} Z_{\delta,\gamma}^* \tau_{\delta,\alpha,w}^6 \quad (2r_D r_T^2 r_V) \quad (13307)$$

$$\tau_{\gamma,\delta,w}^{11} = \sum_{\epsilon \in A} Z_{\epsilon,\delta}^* \tau_{\gamma,\epsilon,w}^{10} \tau_{\gamma,\epsilon,w}^9 \quad (3r_D r_T^3) \quad (13296)$$

$$\tau_{\gamma,\alpha}^8 = \sum_{i \in O} W_{i,\alpha}^3 Y_{i,\gamma}^2 \quad (2r_T r_V N_o) \quad (13308)$$

$$\tau_{\gamma,\delta,w}^{12} = \sum_{\epsilon \in A} Z_{\epsilon,\gamma} \tau_{\epsilon,\delta,w}^{11} \quad (2r_D r_T^3) \quad (13297)$$

$$\tau_{\gamma,\alpha}^9 = \sum_{a \in V} W_{a,\alpha}^4 Y_{a,\gamma}^3 \quad (2r_T r_V N_v) \quad (13309)$$

$${}^2R_{i,\gamma}^4 \leftarrow \sum_{\delta \in A} \sum_{w \in D} \frac{1}{4} {}^2D_{i,w}^4 Y_{i,\delta}^4 \tau_{\delta,\gamma,w}^0 \tau_{\delta,\gamma,w}^{12} \quad (4r_D r_T^2 N_o) \quad (13298)$$

$$\tau_{\gamma,\alpha,i}^{10} = \sum_{\delta \in A} Z_{\gamma,\delta} Y_{i,\delta}^4 \tau_{\delta,\alpha}^9 \quad (3r_T^2 r_V N_o) \quad (13310)$$

$$\tau_{\gamma,\delta,w,i}^{11} = \sum_{\alpha \in B} \tau_{\gamma,\alpha}^8 \tau_{\gamma,\alpha,i}^{10} \tau_{\delta,\alpha,w}^7 \quad (3r_D r_T^2 r_V N_o) \quad (13311)$$

Raw expression

$${}^2R_{j,\zeta}^4 \leftarrow \sum_{\gamma \in A} \sum_{i \in O} \sum_{k \in O} \sum_{l \in O} \sum_{a \in V} \sum_{b \in V} \sum_{c \in V} \sum_{d \in V} \frac{1}{4} Y_{a,\gamma}^{1,*} Y_{i,\gamma}^{2,*} Z_{\gamma,\zeta}^* Y_{b,\zeta}^{3,*} {}^2D_{a,i,b,j} {}^2T_{b,j,a,l} {}^2T_{c,i,d,k} V_{l,d,k,c} \quad (13299)$$

$$\tau_{\gamma,w,i}^{12} = \sum_{\delta \in A} \tau_{\delta,\gamma,w}^0 \tau_{\delta,\gamma,w,i}^{11} \quad (2r_D r_T^2 N_o) \quad (13312)$$

$${}^2R_{i,\gamma}^4 \leftarrow \sum_{w \in D} \frac{1}{4} {}^2D_{i,w}^4 \tau_{\gamma,w,i}^{12} \quad (2r_D r_T N_o) \quad (13313)$$

Factorized expression

$$\tau_{\gamma,\delta,w}^0 = \sum_{a \in V} {}^2D_{a,w}^3 Y_{a,\gamma}^1 Y_{a,\delta}^{3,*} \quad (3r_D r_T^2 N_v) \quad (13300)$$

$$\tau_{\gamma,\delta,w}^1 = \sum_{a \in V} {}^2D_{a,w}^1 Y_{a,\gamma}^3 Y_{a,\delta}^{1,*} \quad (3r_D r_T^2 N_v) \quad (13301)$$

$$\tau_{\gamma,\alpha}^2 = \sum_{a \in V} W_{a,\alpha}^2 Y_{a,\gamma}^1 \quad (2r_T r_V N_v) \quad (13302)$$

$$\tau_{\gamma,\alpha,i}^3 = \sum_{\delta \in A} Y_{i,\delta}^2 Z_{\delta,\gamma} \tau_{\delta,\alpha}^2 \quad (3r_T^2 r_V N_o) \quad (13303)$$

Raw expression

$${}^2R_{j,\zeta}^4 \leftarrow \sum_{\gamma \in A} \sum_{i \in O} \sum_{k \in O} \sum_{l \in O} \sum_{a \in V} \sum_{b \in V} \sum_{c \in V} \sum_{d \in V} \frac{1}{4} Y_{a,\gamma}^{1,*} Y_{i,\gamma}^{2,*} Z_{\gamma,\zeta}^* Y_{b,\zeta}^{3,*} {}^2D_{a,i,b,j} {}^2T_{b,j,a,l} {}^2T_{c,k,d,i} V_{l,c,k,d} \quad (13314)$$

Factorized expression

$$\tau_{\gamma,\delta,w}^0 = \sum_{a \in V} {}^2D_{a,w}^3 Y_{a,\gamma}^1 Y_{a,\delta}^{3,*} \quad (3r_D r_T^2 N_v) \quad (13315)$$

$$\tau_{\gamma,\delta,w,i}^1 = \sum_{\epsilon \in A} Y_{i,\epsilon}^2 Z_{\epsilon,\gamma} \tau_{\epsilon,\delta,w}^0 \quad (3r_D r_T^3 N_o) \quad (13316)$$

$$\tau^2_{\gamma,\delta,w} = \sum_{a \in V} {}^2D^1_{a,w} Y^3_{a,\gamma} Y^{1,*}_{a,\delta} \quad (3r_D r_T^2 N_v) \quad (13317)$$

$$\tau^0_{\gamma,\alpha} = \sum_{a \in V} W^2_{a,\alpha} Y^1_{a,\gamma} \quad (2r_T r_V N_v) \quad (13329)$$

$$\tau^3_{\gamma,\delta,w,i} = \sum_{\epsilon \in A} Y^{2,*}_{i,\epsilon} Z^*_{\epsilon,\delta} \tau^2_{\gamma,\epsilon,w} \quad (3r_D r_T^3 N_o) \quad (13318)$$

$$\tau^1_{\gamma,\alpha,i} = \sum_{\beta \in B} W^1_{i,\beta} X_{\beta,\alpha} \tau^0_{\gamma,\beta} \quad (3r_T r_V^2 N_o) \quad (13330)$$

$$\tau^4_{\gamma,\alpha} = \sum_{a \in V} W^2_{a,\alpha} Y^1_{a,\gamma} \quad (2r_T r_V N_v) \quad (13319)$$

$$\tau^2_{\gamma,\alpha} = \sum_{i \in O} W^3_{i,\alpha} Y^2_{i,\gamma} \quad (2r_T r_V N_o) \quad (13331)$$

$$\tau^5_{\gamma,\alpha,i} = \sum_{\beta \in B} W^1_{i,\beta} X_{\beta,\alpha} \tau^4_{\gamma,\beta} \quad (3r_T r_V^2 N_o) \quad (13320)$$

$$\tau^3_{\gamma,\alpha} = \sum_{a \in V} W^4_{a,\alpha} Y^3_{a,\gamma} \quad (2r_T r_V N_v) \quad (13332)$$

$$\tau^6_{\gamma,\alpha} = \sum_{a \in V} W^4_{a,\alpha} Y^3_{a,\gamma} \quad (2r_T r_V N_v) \quad (13321)$$

$$\tau^4_{\gamma,\delta,i} = \sum_{\alpha \in B} \tau^2_{\gamma,\alpha} \tau^3_{\delta,\alpha} \tau^1_{\gamma,\alpha,i} \quad (3r_T^2 r_V N_o) \quad (13333)$$

$$\tau^7_{\gamma,\alpha,i} = \sum_{\delta \in A} Z_{\gamma,\delta} Y^4_{i,\delta} \tau^6_{\delta,\alpha} \quad (3r_T^2 r_V N_o) \quad (13322)$$

$$\tau^5_{\gamma,i} = \sum_{\delta \in A} Z_{\delta,\gamma} \tau^4_{\delta,\gamma,i} \quad (2r_T^2 N_o) \quad (13334)$$

$$\tau^8_{\gamma,i,j,k} = \sum_{\alpha \in B} W^3_{j,\alpha} \tau^5_{\gamma,\alpha,i} \tau^7_{\gamma,\alpha,k} \quad (3r_T r_V N_o^3) \quad (13323)$$

$$\tau^6_{i,j} = \sum_{\gamma \in A} Y^4_{j,\gamma} \tau^5_{\gamma,i} \quad (2r_T N_o^2) \quad (13335)$$

$$\tau^9_{i,j,k,l} = \sum_{\gamma \in A} Y^2_{k,\gamma} \tau^8_{\gamma,i,j,l} \quad (2r_T N_o^4) \quad (13324)$$

$$\tau^8_{\gamma,\delta,w} = \sum_{a \in V} {}^2D^3_{a,w} Y^1_{a,\gamma} Y^{3,*}_{a,\delta} \quad (3r_D r_T^2 N_v) \quad (13337)$$

$$\tau^{10}_{\gamma,i,j,k} = \sum_{l \in O} Y^4_{l,\gamma} \tau^9_{i,l,j,k} \quad (2r_T N_o^4) \quad (13325)$$

$$\tau^9_{\gamma,\delta,w} = \sum_{a \in V} {}^2D^1_{a,w} Y^3_{a,\gamma} Y^{1,*}_{a,\delta} \quad (3r_D r_T^2 N_v) \quad (13338)$$

$$\tau^{11}_{\gamma,w,i,j} = \sum_{\delta \in A} \sum_{k \in O} \tau^1_{\delta,\gamma,w,k} \tau^{10}_{\delta,k,i,j} \tau^3_{\delta,\gamma,w,j} \quad (3r_D r_T^2 N_o^3) \quad (13326)$$

$$\tau^{10}_{\gamma,\delta,w} = \sum_{i \in O} {}^2D^2_{i,w} Y^4_{i,\gamma} Y^{2,*}_{i,\delta} \quad (3r_D r_T^2 N_o) \quad (13339)$$

$${}^2R^4_{i,\gamma} \leftarrow \sum_{w \in D} \sum_{j \in O} \frac{1}{4} {}^2D^2_{j,w} {}^2D^4_{i,w} \tau^{11}_{\gamma,w,i,j} \quad (3r_D r_T N_o^2) \quad (13327)$$

$$\tau^{11}_{\gamma,\delta,w} = \sum_{\epsilon \in A} Z^*_{\epsilon,\delta} \tau^{10}_{\gamma,\epsilon,w} \tau^9_{\gamma,\epsilon,w} \quad (3r_D r_T^3) \quad (13340)$$

Raw expression

$${}^2R^4_{j,\zeta} \leftarrow \sum_{\gamma \in A} \sum_{i \in O} \sum_{k \in O} \sum_{l \in O} \sum_{a \in V} \sum_{b \in V} \sum_{c \in V} \sum_{d \in V} \frac{1}{4} \quad (13328)$$

$$Y^{1,*}_{a,\gamma} Y^{2,*}_{i,\gamma} Z^*_{\gamma,\zeta} Y^{3,*}_{b,\zeta} {}^2D^{a,i,b,j} {}^2T_{b,j,d,i} {}^2T_{c,k,a,l} V_{k,d,l,c}$$

$$\tau^{12}_{\gamma,\delta,w} = \sum_{\epsilon \in A} Z_{\gamma,\epsilon} \tau^{11}_{\epsilon,\delta,w} \quad (2r_D r_T^3) \quad (13341)$$

$${}^2R^4_{i,\gamma} \leftarrow \sum_{\delta \in A} \sum_{w \in D} \frac{1}{4} {}^2D^4_{i,w} \tau^7_{\delta,i} \tau^{12}_{\delta,\gamma,w} \tau^8_{\delta,\gamma,w} \quad (4r_D r_T^2 N_o) \quad (13342)$$

Factorized expression

Raw expression

$${}^2R^4_{j,\zeta} \leftarrow \sum_{\gamma \in A} \sum_{i \in O} \sum_{k \in O} \sum_{l \in O} \sum_{a \in V} \sum_{b \in V} \sum_{c \in V} \sum_{d \in V} \frac{1}{4} \quad (13343)$$

$$Y^{1,*}_{a,\gamma} \ Y^{2,*}_{i,\gamma} \ Z^*_{\gamma,\zeta} \ Y^{3,*}_{b,\zeta}$$

$${}^2D^{a,i,b,j} \ {}^2T_{b,j,d,l} \ {}^2T_{c,i,a,k} \ V_{k,d,l,c}$$

Factorized expression

$$\tau^0_{\gamma,\alpha} = \sum_{a \in V} W^4_{a,\alpha} Y^1_{a,\gamma} \quad (2r_T r_V N_v) \quad (13344)$$

$$\tau^1_{\gamma,\alpha,i} = \sum_{\beta \in B} X_{\alpha,\beta} W^3_{i,\beta} \tau^0_{\gamma,\beta} \quad (3r_T r_V^2 N_o) \quad (13345)$$

$$\tau^2_{\gamma,\alpha} = \sum_{a \in V} W^2_{a,\alpha} Y^3_{a,\gamma} \quad (2r_T r_V N_v) \quad (13346)$$

$$\tau^3_{\gamma,\alpha,i} = \sum_{\delta \in A} Z_{\gamma,\delta} Y^4_{i,\delta} \tau^2_{\delta,\alpha} \quad (3r_T^2 r_V N_o) \quad (13347)$$

$$\tau^4_{\gamma,i,j,k} = \sum_{\alpha \in B} W^1_{i,\alpha} \tau^1_{\gamma,\alpha} \tau^3_{\gamma,\alpha,k} \quad (3r_T r_V N_o^3) \quad (13348)$$

$$\tau^5_{i,j,k,l} = \sum_{\gamma \in A} Y^2_{k,\gamma} \tau^4_{\gamma,i,j,l} \quad (2r_T N_o^4) \quad (13349)$$

$$\tau^6_{\gamma,i,j,k} = \sum_{l \in O} Y^4_{l,\gamma} \tau^5_{i,l,j,k} \quad (2r_T N_o^4) \quad (13350)$$

$$\tau^7_{\gamma,\delta,w} = \sum_{a \in V} {}^2D^3_{a,w} Y^1_{a,\gamma} Y^{3,*}_{a,\delta} \quad (3r_D r_T^2 N_v) \quad (13351)$$

$$\tau^8_{\gamma,\delta,w,i} = \sum_{\epsilon \in A} Y^2_{i,\epsilon} Z_{\epsilon,\gamma} \tau^7_{\epsilon,\delta,w} \quad (3r_D r_T^3 N_o) \quad (13352)$$

$$\tau^9_{\gamma,\delta,w} = \sum_{a \in V} {}^2D^1_{a,w} Y^3_{a,\gamma} Y^{1,*}_{a,\delta} \quad (3r_D r_T^2 N_v) \quad (13353)$$

$$\tau^{10}_{\gamma,\delta,w,i} = \sum_{\epsilon \in A} Y^{2,*}_{i,\epsilon} Z^*_{\epsilon,\delta} \tau^9_{\gamma,\epsilon,w} \quad (3r_D r_T^3 N_o) \quad (13354)$$

$$\tau^{11}_{\gamma,w,i,j} = \sum_{\delta \in A} \sum_{k \in O} \tau^{10}_{\delta,\gamma,w,i} \tau^6_{\delta,k,i,j} \tau^8_{\delta,\gamma,w,k} \quad (3r_D r_T^2 N_o^3) \quad (13355)$$

$${}^2R^4_{i,\gamma} \leftarrow \sum_{w \in D} \sum_{j \in O} \frac{1}{4} {}^2D^2_{j,w} {}^2D^4_{i,w} \tau^{11}_{\gamma,w,j,i} \quad (3r_D r_T N_o^2) \quad (13356)$$

Raw expression

$${}^2R^4_{j,\zeta} \leftarrow \sum_{\gamma \in A} \sum_{i \in O} \sum_{k \in O} \sum_{l \in O} \sum_{a \in V} \sum_{b \in V} \sum_{c \in V} \sum_{d \in V} \frac{1}{4} \quad (13357)$$

$$Y^{1,*}_{a,\gamma} \ Y^{2,*}_{i,\gamma} \ Z^*_{\gamma,\zeta} \ Y^{3,*}_{b,\zeta}$$

$${}^2D^{a,i,b,j} \ {}^2T_{b,k,a,i} \ {}^2T_{c,j,d,l} \ V_{k,d,l,c}$$

Factorized expression

$$\tau^0_{\gamma,\alpha} = \sum_{a \in V} W^2_{a,\alpha} Y^3_{a,\gamma} \quad (2r_T r_V N_v) \quad (13358)$$

$$\tau^1_{\gamma,\alpha,i} = \sum_{\beta \in B} W^1_{i,\beta} X_{\beta,\alpha} \tau^0_{\gamma,\beta} \quad (3r_T r_V^2 N_o) \quad (13359)$$

$$\tau^2_{\gamma,\alpha} = \sum_{i \in O} W^3_{i,\alpha} Y^4_{i,\gamma} \quad (2r_T r_V N_o) \quad (13360)$$

$$\tau^3_{\gamma,\alpha} = \sum_{\delta \in A} \sum_{i \in O} Y^2_{i,\gamma} Z_{\gamma,\delta} \tau^2_{\delta,\alpha} \tau^1_{\delta,\alpha,i} \quad (4r_T^2 r_V N_o) \quad (13361)$$

$$\tau^4_{\gamma,a} = \sum_{\alpha \in B} W^4_{a,\alpha} \tau^3_{\gamma,\alpha} \quad (2r_T r_V N_v) \quad (13362)$$

$$\tau^5_{\gamma,\delta} = \sum_{a \in V} Y^1_{a,\gamma} \tau^4_{\delta,a} \quad (2r_T^2 N_v) \quad (13363)$$

$$\tau^6_{\gamma,a} = \sum_{\delta \in A} Y^1_{a,\delta} \tau^5_{\gamma,\delta} \quad (2r_T^2 N_v) \quad (13364)$$

$$\tau^7_{\gamma,\delta,w} = \sum_{a \in V} {}^2D^3_{a,w} Y^{3,*}_{a,\delta} \tau^6_{\gamma,a} \quad (3r_D r_T^2 N_v) \quad (13365)$$

$$\tau^8_{\gamma,\delta,w} = \sum_{a \in V} {}^2D^1_{a,w} Y^3_{a,\gamma} Y^{1,*}_{a,\delta} \quad (3r_D r_T^2 N_v) \quad (13366)$$

$$\tau^9_{\gamma,\delta,w} = \sum_{i \in O} {}^2D^2_{i,w} Y^4_{i,\gamma} Y^{2,*}_{i,\delta} \quad (3r_D r_T^2 N_o) \quad (13367)$$

$$\tau^8_{\gamma,\delta,w} = \sum_{a \in V} {}^2D^3_{a,w} Y^1_{a,\gamma} Y^{3,*}_{a,\delta} \quad (3r_D r_T^2 N_v) \quad (13380)$$

$$\tau^{10}_{\gamma,\delta,w} = \sum_{\epsilon \in A} Z^*_{\epsilon,\delta} \tau^8_{\gamma,\epsilon,w} \tau^9_{\gamma,\epsilon,w} \quad (3r_D r_T^3) \quad (13368)$$

$$\tau^9_{\gamma,\delta,w} = \sum_{a \in V} {}^2D^1_{a,w} Y^3_{a,\gamma} Y^{1,*}_{a,\delta} \quad (3r_D r_T^2 N_v) \quad (13381)$$

$$\tau^{11}_{\gamma,\delta,w} = \sum_{\epsilon \in A} Z_{\gamma,\epsilon} \tau^{10}_{\epsilon,\delta,w} \quad (2r_D r_T^3) \quad (13369)$$

$$\tau^{10}_{\gamma,\delta,w} = \sum_{i \in O} {}^2D^2_{i,w} Y^4_{i,\gamma} Y^{2,*}_{i,\delta} \quad (3r_D r_T^2 N_o) \quad (13382)$$

$${}^2R^4_{i,\gamma} \leftarrow \sum_{\delta \in A} \sum_{w \in D} \frac{1}{4} {}^2D^4_{i,w} Y^2_{i,\delta} \tau^{11}_{\delta,\gamma,w} \tau^7_{\delta,\gamma,w} \quad (4r_D r_T^2 N_o) \quad (13370)$$

Raw expression

$$\tau^{11}_{\gamma,\delta,w} = \sum_{\epsilon \in A} Z^*_{\epsilon,\delta} \tau^{10}_{\gamma,\epsilon,w} \tau^9_{\gamma,\epsilon,w} \quad (3r_D r_T^3) \quad (13383)$$

$${}^2R^4_{j,\zeta} \leftarrow \sum_{\gamma \in A} \sum_{i \in O} \sum_{k \in O} \sum_{l \in O} \sum_{a \in V} \sum_{b \in V} \sum_{c \in V} \sum_{d \in V} \frac{1}{4} \quad (13371)$$

$$Y^{1,*}_{a,\gamma} \quad Y^{2,*}_{i,\gamma} \quad Z^*_{\gamma,\zeta} \quad Y^{3,*}_{b,\zeta}$$

$${}^2D^{a,i,b,j} \quad {}^2T_{b,k,a,i} \quad {}^2T_{c,l,d,j} \quad V_{k,c,l,d}$$

$$\tau^{12}_{\gamma,\delta,w} = \sum_{\epsilon \in A} Z_{\gamma,\epsilon} \tau^{11}_{\epsilon,\delta,w} \quad (2r_D r_T^3) \quad (13384)$$

Factorized expression

$${}^2R^4_{i,\gamma} \leftarrow \sum_{\delta \in A} \sum_{w \in D} \frac{1}{4} {}^2D^4_{i,w} \tau^7_{\delta,i} \tau^{12}_{\delta,\gamma,w} \tau^8_{\delta,\gamma,w} \quad (4r_D r_T^2 N_o) \quad (13385)$$

$$\tau^0_{\gamma,\alpha} = \sum_{a \in V} W^2_{a,\alpha} Y^3_{a,\gamma} \quad (2r_T r_V N_v) \quad (13372)$$

Raw expression

$$\tau^1_{\gamma,\alpha,i} = \sum_{\beta \in B} W^1_{i,\beta} X_{\beta,\alpha} \tau^0_{\gamma,\beta} \quad (3r_T r_V^2 N_o) \quad (13373)$$

$${}^2R^4_{j,\zeta} \leftarrow \sum_{\gamma \in A} \sum_{i \in O} \sum_{k \in O} \sum_{l \in O} \sum_{a \in V} \sum_{b \in V} \sum_{c \in V} \sum_{d \in V} \frac{1}{4} \quad (13386)$$

$$Y^{1,*}_{a,\gamma} \quad Y^{2,*}_{i,\gamma} \quad Z^*_{\gamma,\zeta} \quad Y^{3,*}_{b,\zeta}$$

$${}^2D^{a,i,b,j} \quad {}^2T_{b,k,a,l} \quad {}^2T_{c,i,d,j} \quad V_{k,d,l,c}$$

$$\tau^2_{\gamma,\alpha} = \sum_{i \in O} W^3_{i,\alpha} Y^4_{i,\gamma} \quad (2r_T r_V N_o) \quad (13374)$$

Factorized expression

$$\tau^3_{\gamma,\alpha} = \sum_{a \in V} W^4_{a,\alpha} Y^1_{a,\gamma} \quad (2r_T r_V N_v) \quad (13375)$$

$$\tau^0_{\gamma,\alpha} = \sum_{a \in V} W^4_{a,\alpha} Y^1_{a,\gamma} \quad (2r_T r_V N_v) \quad (13387)$$

$$\tau^4_{\gamma,\delta,i} = \sum_{\alpha \in B} \tau^2_{\delta,\alpha} \tau^3_{\gamma,\alpha} \tau^1_{\delta,\alpha,i} \quad (3r_T^2 r_V N_o) \quad (13376)$$

$$\tau^1_{\gamma,\alpha,i} = \sum_{\delta \in A} Y^2_{i,\delta} Z_{\delta,\gamma} \tau^0_{\delta,\alpha} \quad (3r_T^2 r_V N_o) \quad (13388)$$

$$\tau^5_{\gamma,i} = \sum_{\delta \in A} Z_{\gamma,\delta} \tau^4_{\gamma,\delta,i} \quad (2r_T^2 N_o) \quad (13377)$$

$$\tau^2_{\gamma,\alpha} = \sum_{a \in V} W^2_{a,\alpha} Y^3_{a,\gamma} \quad (2r_T r_V N_v) \quad (13389)$$

$$\tau^6_{i,j} = \sum_{\gamma \in A} Y^2_{j,\gamma} \tau^5_{\gamma,i} \quad (2r_T N_o^2) \quad (13378)$$

$$\tau^3_{\gamma,\alpha,i} = \sum_{\beta \in B} W^1_{i,\beta} X_{\beta,\alpha} \tau^2_{\gamma,\beta} \quad (3r_T r_V^2 N_o) \quad (13390)$$

$$\tau^7_{\gamma,i} = \sum_{j \in O} Y^2_{j,\gamma} \tau^6_{j,i} \quad (2r_T N_o^2) \quad (13379)$$

$$\tau^4_{\gamma,\delta,\alpha} = \sum_{i \in O} Y^4_{i,\delta} \tau^3_{\gamma,\alpha,i} \quad (2r_T^2 r_V N_o) \quad (13391)$$



$$\tau_{\gamma,\delta,w}^5 = \sum_{a \in V} {}^2D_{a,w}^3 Y_{a,\gamma}^1 Y_{a,\delta}^{3,*} \quad (3r_D r_T^2 N_v) \quad (13392)$$

$$\tau_{\gamma,\delta,w}^1 = \sum_{a \in V} {}^2D_{a,w}^1 Y_{a,\gamma}^3 Y_{a,\delta}^{1,*} \quad (3r_D r_T^2 N_v) \quad (13403)$$

$$\tau_{\gamma,\delta,w,i}^6 = \sum_{\epsilon \in A} Y_{i,\epsilon}^2 Z_{\epsilon,\gamma} \tau_{\epsilon,\delta,w}^5 \quad (3r_D r_T^3 N_o) \quad (13393)$$

$$\tau_{\gamma,\alpha}^2 = \sum_{a \in V} W_{a,\alpha}^2 Y_{a,\gamma}^1 \quad (2r_T r_V N_v) \quad (13404)$$

$$\tau_{\gamma,\delta,\alpha,w}^7 = \sum_{i \in O} W_{i,\alpha}^3 \tau_{\gamma,\delta,w,i}^6 \quad (2r_D r_T^2 r_V N_o) \quad (13394)$$

$$\tau_{\gamma,\alpha,i}^3 = \sum_{\beta \in B} W_{i,\beta}^1 X_{\beta,\alpha} \tau_{\gamma,\beta}^2 \quad (3r_T r_V^2 N_o) \quad (13405)$$

$$\tau_{\gamma,\delta,w}^8 = \sum_{a \in V} {}^2D_{a,w}^1 Y_{a,\gamma}^3 Y_{a,\delta}^{1,*} \quad (3r_D r_T^2 N_v) \quad (13395)$$

$$\tau_{\gamma,\alpha}^4 = \sum_{i \in O} W_{i,\alpha}^3 Y_{i,\gamma}^2 \quad (2r_T r_V N_o) \quad (13406)$$

$$\tau_{\gamma,\alpha}^5 = \sum_{a \in V} W_{a,\alpha}^4 Y_{a,\gamma}^3 \quad (2r_T r_V N_v) \quad (13407)$$

$$\tau_{\gamma,\delta,w,i}^9 = \sum_{\epsilon \in A} Y_{i,\epsilon}^{2,*} Z_{\epsilon,\delta}^* \tau_{\gamma,\epsilon,w}^8 \quad (3r_D r_T^3 N_o) \quad (13396)$$

$$\tau_{\gamma,\delta,i}^6 = \sum_{\alpha \in B} \tau_{\gamma,\alpha}^4 \tau_{\delta,\alpha}^5 \tau_{\gamma,\alpha,i}^3 \quad (3r_T^2 r_V N_o) \quad (13408)$$

$$\tau_{\gamma,\delta,\epsilon,w}^{10} = \sum_{i \in O} {}^2D_{i,w}^2 Y_{i,\delta}^4 \tau_{\gamma,\epsilon,w,i}^9 \quad (3r_D r_T^3 N_o) \quad (13397)$$

$$\tau_{\gamma,i}^7 = \sum_{\delta \in A} Z_{\delta,\gamma} \tau_{\delta,\gamma,i}^6 \quad (2r_T^2 N_o) \quad (13409)$$

$$\tau_{i,j}^8 = \sum_{\gamma \in A} Y_{j,\gamma}^4 \tau_{\gamma,i}^7 \quad (2r_T N_o^2) \quad (13410)$$

$$\tau_{\gamma,\delta,\alpha,w}^{11} = \sum_{\epsilon \in A} \tau_{\epsilon,\gamma,\alpha}^4 \tau_{\gamma,\epsilon,\delta,w}^{10} \tau_{\epsilon,\delta,\alpha,w}^7 \quad (3r_D r_T^3 r_V) \quad (13398)$$

$$\tau_{\gamma,i}^9 = \sum_{j \in O} Y_{j,\gamma}^4 \tau_{j,i}^8 \quad (2r_T N_o^2) \quad (13411)$$

$$\tau_{\gamma,w,i}^{12} = \sum_{\delta \in A} \sum_{\alpha \in B} \tau_{\delta,\alpha,i}^1 \tau_{\delta,\gamma,\alpha,w}^{11} \quad (2r_D r_T^2 r_V N_o) \quad (13399)$$

$$\tau_{\gamma,\delta,w}^{10} = \sum_{i \in O} {}^2D_{i,w}^2 Y_{i,\delta}^{2,*} \tau_{\gamma,i}^9 \quad (3r_D r_T^2 N_o) \quad (13412)$$

$$\tau_{\gamma,\delta,w}^{11} = \sum_{\epsilon \in A} Z_{\epsilon,\delta}^* \tau_{\gamma,\epsilon,w}^1 \tau_{\gamma,\epsilon,w}^{10} \quad (3r_D r_T^3) \quad (13413)$$

$${}^2R_{i,\gamma}^4 \leftarrow \sum_{w \in D} \frac{1}{4} {}^2D_{i,w}^4 \tau_{\gamma,w,i}^{12} \quad (2r_D r_T N_o) \quad (13400)$$

$$\tau_{\gamma,\delta,w}^{12} = \sum_{\epsilon \in A} Z_{\gamma,\epsilon} \tau_{\epsilon,\delta,w}^{11} \quad (2r_D r_T^3) \quad (13414)$$

Raw expression

$${}^2R_{j,\zeta}^4 \leftarrow \sum_{\gamma \in A} \sum_{i \in O} \sum_{k \in O} \sum_{l \in O} \sum_{a \in V} \sum_{b \in V} \sum_{c \in V} \sum_{d \in V} \frac{1}{4} \quad (13401)$$

$$Y_{a,\gamma}^{1,*} Y_{i,\gamma}^{2,*} Z_{\gamma,\zeta}^* Y_{b,\zeta}^{3,*} {}^2D_{a,i,b,j} {}^2T_{b,k,a,l} {}^2T_{c,j,d,i} V_{k,c,l,d}$$

$${}^2R_{i,\gamma}^4 \leftarrow \sum_{\delta \in A} \sum_{w \in D} \frac{1}{4} {}^2D_{i,w}^4 Y_{i,\delta}^2 \tau_{\delta,\gamma,w}^0 \tau_{\delta,\gamma,w}^{12} \quad (4r_D r_T^2 N_o) \quad (13415)$$

Raw expression

Factorized expression

$$\tau_{\gamma,\delta,w}^0 = \sum_{a \in V} {}^2D_{a,w}^3 Y_{a,\gamma}^1 Y_{a,\delta}^{3,*} \quad (3r_D r_T^2 N_v) \quad (13402)$$

$${}^2R_{j,\zeta}^4 \leftarrow \sum_{\gamma \in A} \sum_{i \in O} \sum_{k \in O} \sum_{l \in O} \sum_{a \in V} \sum_{b \in V} \sum_{c \in V} \sum_{d \in V} \frac{1}{4} \quad (13416)$$

$$Y_{a,\gamma}^{1,*} Y_{i,\gamma}^{2,*} Z_{\gamma,\zeta}^* Y_{b,\zeta}^{3,*} {}^2D_{a,i,b,j} {}^2T_{b,k,c,i} {}^2T_{d,j,a,l} V_{l,c,k,d}$$

Factorized expression

$$\tau^0_{\gamma,\delta,w} = \sum_{a \in V} {}^2D^3_{a,w} Y^1_{a,\gamma} Y^{3,*}_{a,\delta} \quad (3r_D r_T^2 N_v) \quad (13417)$$

$$\tau^1_{\gamma,\delta,w} = \sum_{a \in V} {}^2D^1_{a,w} Y^3_{a,\gamma} Y^{1,*}_{a,\delta} \quad (3r_D r_T^2 N_v) \quad (13418)$$

$$\tau^2_{\gamma,\alpha} = \sum_{a \in V} W^2_{a,\alpha} Y^3_{a,\gamma} \quad (2r_T r_V N_v) \quad (13419)$$

$$\tau^3_{\gamma,\alpha,i} = \sum_{\beta \in B} W^1_{i,\beta} X_{\beta,\alpha} \tau^2_{\gamma,\beta} \quad (3r_T r_V^2 N_o) \quad (13420)$$

$$\tau^4_{\gamma,\alpha} = \sum_{i \in O} W^3_{i,\alpha} Y^4_{i,\gamma} \quad (2r_T r_V N_o) \quad (13421)$$

$$\tau^5_{\gamma,\alpha} = \sum_{a \in V} W^4_{a,\alpha} Y^1_{a,\gamma} \quad (2r_T r_V N_v) \quad (13422)$$

$$\tau^6_{\gamma,\delta,i} = \sum_{\alpha \in B} \tau^4_{\delta,\alpha} \tau^5_{\gamma,\alpha} \tau^3_{\delta,\alpha,i} \quad (3r_T^2 r_V N_o) \quad (13423)$$

$$\tau^7_{\gamma,i} = \sum_{\delta \in A} Z_{\gamma,\delta} \tau^6_{\gamma,\delta,i} \quad (2r_T^2 N_o) \quad (13424)$$

$$\tau^8_{i,j} = \sum_{\gamma \in A} Y^2_{j,\gamma} \tau^7_{\gamma,i} \quad (2r_T N_o^2) \quad (13425)$$

$$\tau^9_{\gamma,i} = \sum_{j \in O} Y^4_{j,\gamma} \tau^8_{j,i} \quad (2r_T N_o^2) \quad (13426)$$

$$\tau^{10}_{\gamma,\delta,w} = \sum_{i \in O} {}^2D^2_{i,w} Y^{2,*}_{i,\delta} \tau^9_{\gamma,i} \quad (3r_D r_T^2 N_o) \quad (13427)$$

$$\tau^{11}_{\gamma,\delta,w} = \sum_{\epsilon \in A} Z^*_{\epsilon,\delta} \tau^1_{\gamma,\epsilon,w} \tau^{10}_{\gamma,\epsilon,w} \quad (3r_D r_T^3) \quad (13428)$$

$$\tau^{12}_{\gamma,\delta,w} = \sum_{\epsilon \in A} Z_{\gamma,\epsilon} \tau^{11}_{\epsilon,\delta,w} \quad (2r_D r_T^3) \quad (13429)$$

$${}^2R^4_{i,\gamma} \leftarrow \sum_{\delta \in A} \sum_{w \in D} \frac{1}{4} {}^2D^4_{i,w} Y^2_{i,\delta} \tau^0_{\delta,\gamma,w} \tau^{12}_{\delta,\gamma,w} \quad (4r_D r_T^2 N_o) \quad (13430)$$

Raw expression

$${}^2R^4_{j,\zeta} \leftarrow \sum_{\gamma \in A} \sum_{i \in O} \sum_{k \in O} \sum_{l \in O} \sum_{a \in V} \sum_{b \in V} \sum_{c \in V} \sum_{d \in V} \frac{1}{4} \quad (13431)$$

$$Y^{1,*}_{a,\gamma} Y^{2,*}_{i,\gamma} Z^*_{\gamma,\zeta} Y^{3,*}_{b,\zeta} {}^2D^{a,i,b,j} {}^2T_{b,k,c,l} {}^2T_{d,j,a,i} V_{k,c,l,d}$$

Factorized expression

$$\tau^0_{\gamma,\delta,w} = \sum_{a \in V} {}^2D^1_{a,w} Y^3_{a,\gamma} Y^{1,*}_{a,\delta} \quad (3r_D r_T^2 N_v) \quad (13432)$$

$$\tau^1_{\gamma,\alpha} = \sum_{a \in V} W^2_{a,\alpha} Y^3_{a,\gamma} \quad (2r_T r_V N_v) \quad (13433)$$

$$\tau^2_{\gamma,\alpha,i} = \sum_{\beta \in B} W^1_{i,\beta} X_{\beta,\alpha} \tau^1_{\gamma,\beta} \quad (3r_T r_V^2 N_o) \quad (13434)$$

$$\tau^3_{\gamma,\alpha} = \sum_{i \in O} W^3_{i,\alpha} Y^4_{i,\gamma} \quad (2r_T r_V N_o) \quad (13435)$$

$$\tau^4_{\gamma,\alpha} = \sum_{a \in V} W^4_{a,\alpha} Y^1_{a,\gamma} \quad (2r_T r_V N_v) \quad (13436)$$

$$\tau^5_{\gamma,\delta,i} = \sum_{\alpha \in B} \tau^3_{\delta,\alpha} \tau^4_{\gamma,\alpha} \tau^2_{\delta,\alpha,i} \quad (3r_T^2 r_V N_o) \quad (13437)$$

$$\tau^6_{\gamma,\delta,\epsilon} = \sum_{i \in O} Z_{\gamma,\delta} Y^4_{i,\delta} \tau^5_{\gamma,\epsilon,i} \quad (3r_T^3 N_o) \quad (13438)$$

$$\tau^7_{\gamma,\delta,i} = \sum_{\epsilon \in A} Y^2_{i,\epsilon} \tau^6_{\epsilon,\gamma,\delta} \quad (2r_T^3 N_o) \quad (13439)$$

$$\tau^8_{\gamma,\delta,w} = \sum_{\epsilon \in A} \sum_{i \in O} {}^2D^2_{i,w} Y^{2,*}_{i,\delta} \tau^0_{\epsilon,\delta,w} \tau^7_{\epsilon,\gamma,i} \quad (4r_D r_T^3 N_o) \quad (13440)$$

$$\tau^9_{\gamma,\delta,w} = \sum_{\epsilon \in A} Z^*_{\epsilon,\delta} \tau^8_{\gamma,\epsilon,w} \quad (2r_D r_T^3) \quad (13441)$$

$$\tau^{10}_{\gamma,\delta,w} = \sum_{\epsilon \in A} Z_{\gamma,\epsilon} \tau^9_{\epsilon,\delta,w} \quad (2r_D r_T^3) \quad (13442)$$

$$\tau^{11}_{\gamma,\delta,w} = \sum_{a \in V} {}^2D^3_{a,w} Y^1_{a,\gamma} Y^{3,*}_{a,\delta} \quad (3r_D r_T^2 N_v) \quad (13443)$$

$${}^2R^4_{i,\gamma} \leftarrow \sum_{\delta \in A} \sum_{w \in D} \frac{1}{4} {}^2D^4_{i,w} Y^2_{i,\delta} \tau^{10}_{\delta,\gamma,w} \tau^{11}_{\delta,\gamma,w} \quad (4r_D r_T^2 N_o) \quad \tau^{10}_{\gamma,\delta,w} = \sum_{\epsilon \in A} Z^*_{\epsilon,\delta} \tau^8_{\gamma,\epsilon,w} \tau^9_{\gamma,\epsilon,w} \quad (3r_D r_T^3) \quad (13444)$$

Raw expression

$$\tau^{11}_{\gamma,\delta,w} = \sum_{\epsilon \in A} Z_{\gamma,\epsilon} \tau^{10}_{\epsilon,\delta,w} \quad (2r_D r_T^3) \quad (13457)$$

$${}^2R^4_{j,\zeta} \leftarrow \sum_{\gamma \in A} \sum_{i \in O} \sum_{k \in O} \sum_{l \in O} \sum_{a \in V} \sum_{b \in V} \sum_{c \in V} \sum_{d \in V} \frac{1}{4} \quad (13445)$$

$$Y^{1,*}_{a,\gamma} \quad Y^{2,*}_{i,\gamma} \quad Z^*_{\gamma,\zeta} \quad Y^{3,*}_{b,\zeta}$$

$${}^2D^{a,i,b,j} \quad {}^2T_{b,l,d,j} \quad {}^2T_{c,i,a,k} \quad V_{k,c,l,d}$$

$${}^2R^4_{i,\gamma} \leftarrow \sum_{\delta \in A} \sum_{w \in D} \frac{1}{4} {}^2D^4_{i,w} Y^2_{i,\delta} \tau^0_{\delta,\gamma,w} \tau^{11}_{\delta,\gamma,w} \quad (4r_D r_T^2 N_o) \quad (13458)$$

Factorized expression

Raw expression

$$\tau^0_{\gamma,\delta,w} = \sum_{a \in V} {}^2D^3_{a,w} Y^1_{a,\gamma} Y^{3,*}_{a,\delta} \quad (3r_D r_T^2 N_v) \quad (13446)$$

$${}^2R^4_{j,\zeta} \leftarrow \sum_{\gamma \in A} \sum_{i \in O} \sum_{k \in O} \sum_{l \in O} \sum_{a \in V} \sum_{b \in V} \sum_{c \in V} \sum_{d \in V} \frac{1}{4} \quad (13459)$$

$$Y^{1,*}_{a,\gamma} \quad Y^{2,*}_{i,\gamma} \quad Z^*_{\gamma,\zeta} \quad Y^{3,*}_{b,\zeta}$$

$${}^2D^{a,i,b,j} \quad {}^2T_{b,l,d,j} \quad {}^2T_{c,k,a,i} \quad V_{k,d,l,c}$$

$$\tau^1_{\gamma,\alpha} = \sum_{a \in V} W^4_{a,\alpha} Y^1_{a,\gamma} \quad (2r_T r_V N_v) \quad (13447)$$

Factorized expression

$$\tau^2_{\gamma,\alpha,i} = \sum_{\beta \in B} X_{\alpha,\beta} W^3_{i,\beta} \tau^1_{\gamma,\beta} \quad (3r_T r_V^2 N_o) \quad (13448)$$

$$\tau^0_{\gamma,\delta,w} = \sum_{a \in V} {}^2D^1_{a,w} Y^3_{a,\gamma} Y^{1,*}_{a,\delta} \quad (3r_D r_T^2 N_v) \quad (13460)$$

$$\tau^3_{\gamma,\alpha} = \sum_{i \in O} W^1_{i,\alpha} Y^2_{i,\gamma} \quad (2r_T r_V N_o) \quad (13449)$$

$$\tau^1_{\gamma,\delta,w} = \sum_{i \in O} {}^2D^2_{i,w} Y^4_{i,\gamma} Y^{2,*}_{i,\delta} \quad (3r_D r_T^2 N_o) \quad (13461)$$

$$\tau^4_{\gamma,\alpha} = \sum_{\delta \in A} \sum_{i \in O} Z_{\delta,\gamma} Y^4_{i,\gamma} \tau^3_{\delta,\alpha} \tau^2_{\delta,\alpha,i} \quad (4r_T^2 r_V N_o) \quad (13450)$$

$$\tau^2_{\gamma,\delta,w} = \sum_{\epsilon \in A} Z^*_{\epsilon,\delta} \tau^0_{\gamma,\epsilon,w} \tau^1_{\gamma,\epsilon,w} \quad (3r_D r_T^3) \quad (13462)$$

$$\tau^5_{\gamma,a} = \sum_{\alpha \in B} W^2_{a,\alpha} \tau^4_{\gamma,\alpha} \quad (2r_T r_V N_v) \quad (13451)$$

$$\tau^3_{\gamma,\delta,w} = \sum_{\epsilon \in A} Z_{\gamma,\epsilon} \tau^2_{\epsilon,\delta,w} \quad (2r_D r_T^3) \quad (13463)$$

$$\tau^6_{a,b} = \sum_{\gamma \in A} Y^3_{b,\gamma} \tau^5_{\gamma,a} \quad (2r_T N_v^2) \quad (13452)$$

$$\tau^4_{\gamma,\alpha} = \sum_{a \in V} W^4_{a,\alpha} Y^1_{a,\gamma} \quad (2r_T r_V N_v) \quad (13464)$$

$$\tau^7_{\gamma,a} = \sum_{b \in V} Y^3_{b,\gamma} \tau^6_{b,a} \quad (2r_T N_v^2) \quad (13453)$$

$$\tau^5_{\gamma,\alpha,i} = \sum_{\beta \in B} X_{\alpha,\beta} W^3_{i,\beta} \tau^4_{\gamma,\beta} \quad (3r_T r_V^2 N_o) \quad (13465)$$

$$\tau^8_{\gamma,\delta,w} = \sum_{a \in V} {}^2D^1_{a,w} Y^{1,*}_{a,\delta} \tau^7_{\gamma,a} \quad (3r_D r_T^2 N_v) \quad (13454)$$

$$\tau^6_{\gamma,\alpha} = \sum_{i \in O} W^1_{i,\alpha} Y^2_{i,\gamma} \quad (2r_T r_V N_o) \quad (13466)$$

$$\tau^7_{\gamma,\alpha} = \sum_{a \in V} W^2_{a,\alpha} Y^3_{a,\gamma} \quad (2r_T r_V N_v) \quad (13467)$$

$$\tau^9_{\gamma,\delta,w} = \sum_{i \in O} {}^2D^2_{i,w} Y^4_{i,\gamma} Y^{2,*}_{i,\delta} \quad (3r_D r_T^2 N_o) \quad (13455)$$

$$\tau^8_{\gamma,\delta,i} = \sum_{\alpha \in B} \tau^6_{\gamma,\alpha} \tau^7_{\delta,\alpha} \tau^5_{\gamma,\alpha,i} \quad (3r_T^2 r_V N_o) \quad (13468)$$

$$\tau_{\gamma,\delta,\epsilon}^9 = \sum_{i \in O} Y_{i,\delta}^2 Z_{\delta,\epsilon} \tau_{\gamma,\epsilon,i}^8 \quad (3r_T^3 N_o) \quad (13469)$$

$$\tau_{\gamma,\delta,i}^{10} = \sum_{\epsilon \in A} Y_{i,\epsilon}^4 \tau_{\gamma,\delta,\epsilon}^9 \quad (2r_T^3 N_o) \quad (13470)$$

$$\tau_{\gamma,\delta,w,i}^{11} = \sum_{\epsilon \in A} \tau_{\epsilon,\gamma,i}^{10} \tau_{\epsilon,\delta,w}^3 \quad (2r_D r_T^3 N_o) \quad (13471)$$

$$\tau_{\gamma,\delta,w}^{12} = \sum_{a \in V} {}^2D_{a,w}^3 Y_{a,\gamma}^1 Y_{a,\delta}^{3,*} \quad (3r_D r_T^2 N_v) \quad (13472)$$

$$\tau_{\gamma,w,i}^{13} = \sum_{\delta \in A} \tau_{\delta,\gamma,w}^{12} \tau_{\delta,\gamma,w,i}^{11} \quad (2r_D r_T^2 N_o) \quad (13473)$$

$${}^2R_{i,\gamma}^4 \leftarrow \sum_{w \in D} \frac{1}{4} {}^2D_{i,w}^4 \tau_{\gamma,w,i}^{13} \quad (2r_D r_T N_o) \quad (13474)$$

Raw expression

$${}^2R_{j,\zeta}^4 \leftarrow \sum_{\gamma \in A} \sum_{i \in O} \sum_{k \in O} \sum_{l \in O} \sum_{a \in V} \sum_{b \in V} \sum_{c \in V} \sum_{d \in V} \frac{1}{4} \quad (13475)$$

$$Y_{a,\gamma}^{1,*} Y_{i,\gamma}^{2,*} Z_{\gamma,\zeta}^* Y_{b,\zeta}^{3,*} {}^2D_{a,i,b,j} {}^2T_{c,i,a,k} {}^2T_{d,j,b,l} V_{k,c,l,d}$$

Factorized expression

$$\tau_{\gamma,\alpha}^0 = \sum_{a \in V} W_{a,\alpha}^4 Y_{a,\gamma}^1 \quad (2r_T r_V N_v) \quad (13476)$$

$$\tau_{\gamma,\alpha,i}^1 = \sum_{\delta \in A} Y_{i,\delta}^2 Z_{\delta,\gamma} \tau_{\delta,\alpha}^0 \quad (3r_T^2 r_V N_o) \quad (13477)$$

$$\tau_{\gamma,\alpha}^2 = \sum_{a \in V} W_{a,\alpha}^2 Y_{a,\gamma}^1 \quad (2r_T r_V N_v) \quad (13478)$$

$$\tau_{\gamma,\alpha,i}^3 = \sum_{\beta \in B} W_{i,\beta}^1 X_{\beta,\alpha} \tau_{\gamma,\beta}^2 \quad (3r_T r_V^2 N_o) \quad (13479)$$

$$\tau_{\gamma,\delta,\alpha}^4 = \sum_{i \in O} Y_{i,\delta}^4 \tau_{\gamma,\alpha,i}^3 \quad (2r_T^2 r_V N_o) \quad (13480)$$

$$\tau_{\gamma,\delta,w}^5 = \sum_{a \in V} {}^2D_{a,w}^3 Y_{a,\gamma}^3 Y_{a,\delta}^{3,*} \quad (3r_D r_T^2 N_v) \quad (13481)$$

$$\tau_{\gamma,\delta,w,i}^6 = \sum_{\epsilon \in A} Z_{\gamma,\epsilon} Y_{i,\epsilon}^4 \tau_{\epsilon,\delta,w}^5 \quad (3r_D r_T^3 N_o) \quad (13482)$$

$$\tau_{\gamma,\delta,\alpha,w}^7 = \sum_{i \in O} W_{i,\alpha}^3 \tau_{\gamma,\delta,w,i}^6 \quad (2r_D r_T^2 r_V N_o) \quad (13483)$$

$$\tau_{\gamma,\delta,w}^8 = \sum_{a \in V} {}^2D_{a,w}^1 Y_{a,\gamma}^3 Y_{a,\delta}^{1,*} \quad (3r_D r_T^2 N_v) \quad (13484)$$

$$\tau_{\gamma,\delta,w,i}^9 = \sum_{\epsilon \in A} Y_{i,\epsilon}^{2,*} Z_{\epsilon,\delta}^* \tau_{\gamma,\epsilon,w}^8 \quad (3r_D r_T^3 N_o) \quad (13485)$$

$$\tau_{\gamma,\delta,\epsilon,w}^{10} = \sum_{i \in O} {}^2D_{i,w}^2 Y_{i,\gamma}^2 \tau_{\delta,\epsilon,w,i}^9 \quad (3r_D r_T^3 N_o) \quad (13486)$$

$$\tau_{\gamma,\delta,\alpha,w}^{11} = \sum_{\epsilon \in A} \tau_{\epsilon,\gamma,\alpha}^4 \tau_{\epsilon,\gamma,\delta,w}^{10} \tau_{\epsilon,\delta,\alpha,w}^7 \quad (3r_D r_T^3 r_V) \quad (13487)$$

$$\tau_{\gamma,w,i}^{12} = \sum_{\delta \in A} \sum_{\alpha \in B} \tau_{\delta,\alpha,i}^1 \tau_{\delta,\gamma,\alpha,w}^{11} \quad (2r_D r_T^2 r_V N_o) \quad (13488)$$

$${}^2R_{i,\gamma}^4 \leftarrow \sum_{w \in D} \frac{1}{4} {}^2D_{i,w}^4 \tau_{\gamma,w,i}^{12} \quad (2r_D r_T N_o) \quad (13489)$$

Raw expression

$${}^2R_{j,\zeta}^4 \leftarrow \sum_{\gamma \in A} \sum_{i \in O} \sum_{k \in O} \sum_{l \in O} \sum_{a \in V} \sum_{b \in V} \sum_{c \in V} \sum_{d \in V} \frac{1}{4} \quad (13490)$$

$$Y_{a,\gamma}^{1,*} Y_{i,\gamma}^{2,*} Z_{\gamma,\zeta}^* Y_{b,\zeta}^{3,*} {}^2D_{a,i,b,j} {}^2T_{c,i,a,k} {}^2T_{d,l,b,j} V_{k,d,l,c}$$

Factorized expression

$$\tau_{\gamma,\delta,w}^0 = \sum_{a \in V} {}^2D_{a,w}^1 Y_{a,\gamma}^3 Y_{a,\delta}^{1,*} \quad (3r_D r_T^2 N_v) \quad (13491)$$

$$\tau_{\gamma,\alpha}^1 = \sum_{a \in V} W_{a,\alpha}^2 Y_{a,\gamma}^1 \quad (2r_T r_V N_v) \quad (13492)$$

$$\tau_{\gamma,\alpha,i}^2 = \sum_{\delta \in A} Y_{i,\delta}^2 Z_{\delta,\gamma} \tau_{\delta,\alpha}^1 \quad (3r_T^2 r_V N_o) \quad (13493)$$

$$\tau^3_{\gamma,\alpha} = \sum_{i \in O} W^1_{i,\alpha} Y^4_{i,\gamma} \quad (2r_T r_V N_o) \quad (13494)$$

$$\tau^0_{\gamma,\delta,w} = \sum_{a \in V} {}^2D^3_{a,w} Y^3_{a,\gamma} Y^{3,*}_{a,\delta} \quad (3r_D r_T^2 N_v) \quad (13506)$$

$$\tau^4_{\gamma,\alpha,w} = \sum_{\delta \in A} \sum_{i \in O} {}^2D^2_{i,w} Y^{2,*}_{i,\gamma} \tau^3_{\delta,\alpha} \tau^0_{\delta,\gamma,w} \tau^2_{\delta,\alpha,i} \quad (5r_D r_T^2 r_V N_o) \quad (13495)$$

$$\tau^1_{\gamma,\delta,w} = \sum_{i \in O} {}^2D^2_{i,w} Y^2_{i,\gamma} Y^{2,*}_{i,\delta} \quad (3r_D r_T^2 N_o) \quad (13507)$$

$$\tau^5_{\gamma,\alpha,w} = \sum_{\beta \in B} X_{\beta,\alpha} \tau^4_{\gamma,\beta,w} \quad (2r_D r_T r_V^2) \quad (13496)$$

$$\tau^2_{\gamma,\alpha} = \sum_{a \in V} W^4_{a,\alpha} Y^1_{a,\gamma} \quad (2r_T r_V N_v) \quad (13508)$$

$$\tau^6_{\gamma,\alpha,w} = \sum_{\delta \in A} Z^*_{\delta,\gamma} \tau^5_{\delta,\alpha,w} \quad (2r_D r_T^2 r_V) \quad (13497)$$

$$\tau^3_{\gamma,\alpha,i} = \sum_{\beta \in B} X_{\alpha,\beta} W^3_{i,\beta} \tau^2_{\gamma,\beta} \quad (3r_T r_V^2 N_o) \quad (13509)$$

$$\tau^7_{\gamma,\alpha} = \sum_{a \in V} W^4_{a,\alpha} Y^1_{a,\gamma} \quad (2r_T r_V N_v) \quad (13498)$$

$$\tau^4_{\gamma,\alpha} = \sum_{i \in O} W^1_{i,\alpha} Y^2_{i,\gamma} \quad (2r_T r_V N_o) \quad (13510)$$

$$\tau^8_{\gamma,\alpha,i} = \sum_{\delta \in A} Y^2_{i,\delta} Z_{\delta,\gamma} \tau^7_{\delta,\alpha} \quad (3r_T^2 r_V N_o) \quad (13499)$$

$$\tau^5_{\gamma,\alpha} = \sum_{\delta \in A} \sum_{i \in O} Z_{\delta,\gamma} Y^4_{i,\gamma} \tau^4_{\delta,\alpha} \tau^3_{\delta,\alpha,i} \quad (4r_T^2 r_V N_o) \quad (13511)$$

$$\tau^9_{\gamma,\alpha} = \sum_{i \in O} W^3_{i,\alpha} Y^4_{i,\gamma} \quad (2r_T r_V N_o) \quad (13500)$$

$$\tau^6_{\gamma,a} = \sum_{\alpha \in B} W^2_{a,\alpha} \tau^5_{\gamma,\alpha} \quad (2r_T r_V N_v) \quad (13512)$$

$$\tau^{10}_{\gamma,\delta,w,i} = \sum_{\alpha \in B} \tau^9_{\gamma,\alpha} \tau^6_{\delta,\alpha,w} \tau^8_{\gamma,\alpha,i} \quad (3r_D r_T^2 r_V N_o) \quad (13501)$$

$$\tau^7_{a,b} = \sum_{\gamma \in A} Y^3_{b,\gamma} \tau^6_{\gamma,a} \quad (2r_T N_v^2) \quad (13513)$$

$$\tau^{11}_{\gamma,\delta,w} = \sum_{a \in V} {}^2D^3_{a,w} Y^3_{a,\gamma} Y^{3,*}_{a,\delta} \quad (3r_D r_T^2 N_v) \quad (13502)$$

$$\tau^8_{\gamma,a} = \sum_{b \in V} Y^1_{b,\gamma} \tau^7_{b,a} \quad (2r_T N_v^2) \quad (13514)$$

$$\tau^{12}_{\gamma,w,i} = \sum_{\delta \in A} \tau^{11}_{\delta,\gamma,w} \tau^{10}_{\delta,\gamma,w,i} \quad (2r_D r_T^2 N_o) \quad (13503)$$

$$\tau^9_{\gamma,\delta,w} = \sum_{a \in V} {}^2D^1_{a,w} Y^{1,*}_{a,\delta} \tau^8_{\gamma,a} \quad (3r_D r_T^2 N_v) \quad (13515)$$

$${}^2R^4_{i,\gamma} \leftarrow \sum_{w \in D} \frac{1}{4} {}^2D^4_{i,w} \tau^{12}_{\gamma,w,i} \quad (2r_D r_T N_o) \quad (13504)$$

$$\tau^{10}_{\gamma,\delta,w} = \sum_{\epsilon \in A} Z^*_{\epsilon,\delta} \tau^1_{\gamma,\epsilon,w} \tau^9_{\gamma,\epsilon,w} \quad (3r_D r_T^3) \quad (13516)$$

Raw expression

$$\tau^{11}_{\gamma,\delta,w} = \sum_{\epsilon \in A} Z_{\epsilon,\gamma} \tau^{10}_{\epsilon,\delta,w} \quad (2r_D r_T^3) \quad (13517)$$

$${}^2R^4_{j,\zeta} \leftarrow \sum_{\gamma \in A} \sum_{i \in O} \sum_{k \in O} \sum_{l \in O} \sum_{a \in V} \sum_{b \in V} \sum_{c \in V} \sum_{d \in V} \frac{1}{4} \quad (13505)$$

$$Y^{1,*}_{a,\gamma} Y^{2,*}_{i,\gamma} Z^*_{\gamma,\zeta} Y^{3,*}_{b,\zeta} {}^2D^{a,i,b,j} {}^2T_{c,i,b,k} {}^2T_{d,j,a,l} V_{l,c,k,d}$$

Factorized expression

$${}^2R^4_{i,\gamma} \leftarrow \sum_{\delta \in A} \sum_{w \in D} \frac{1}{4} {}^2D^4_{i,w} Y^4_{i,\delta} \tau^0_{\delta,\gamma,w} \tau^{11}_{\delta,\gamma,w} \quad (4r_D r_T^2 N_o) \quad (13518)$$

Raw expression

$${}^2R^4_{j,\zeta} \leftarrow \sum_{\gamma \in A} \sum_{i \in O} \sum_{k \in O} \sum_{l \in O} \sum_{a \in V} \sum_{b \in V} \sum_{c \in V} \sum_{d \in V} \frac{1}{4} \quad (13519)$$

$$Y^{1,*}_{a,\gamma} \ Y^{2,*}_{i,\gamma} \ Z^*_{\gamma,\zeta} \ Y^{3,*}_{b,\zeta}$$

$${}^2D^{a,i,b,j} \ {}^2T_{c,k,a,i} \ {}^2T_{d,j,b,l} \ V_{k,d,l,c}$$

Factorized expression

$$\tau^0_{\gamma,\delta,w} = \sum_{a \in V} {}^2D^1_{a,w} Y^3_{a,\gamma} Y^{1,*}_{a,\delta} \quad (3r_D r_T^2 N_v) \quad (13520)$$

$$\tau^1_{\gamma,\alpha} = \sum_{a \in V} W^2_{a,\alpha} Y^1_{a,\gamma} \quad (2r_T r_V N_v) \quad (13521)$$

$$\tau^2_{\gamma,\alpha,i} = \sum_{\beta \in B} W^1_{i,\beta} X_{\beta,\alpha} \tau^1_{\gamma,\beta} \quad (3r_T r_V^2 N_o) \quad (13522)$$

$$\tau^3_{\gamma,\alpha} = \sum_{i \in O} W^3_{i,\alpha} Y^2_{i,\gamma} \quad (2r_T r_V N_o) \quad (13523)$$

$$\tau^4_{\gamma,\alpha} = \sum_{a \in V} W^4_{a,\alpha} Y^1_{a,\gamma} \quad (2r_T r_V N_v) \quad (13524)$$

$$\tau^5_{\gamma,\delta,i} = \sum_{\alpha \in B} \tau^3_{\gamma,\alpha} \tau^4_{\delta,\alpha} \tau^2_{\gamma,\alpha,i} \quad (3r_T^2 r_V N_o) \quad (13525)$$

$$\tau^6_{\gamma,\delta,\epsilon} = \sum_{i \in O} Z_{\delta,\epsilon} Y^4_{i,\epsilon} \tau^5_{\gamma,\delta,i} \quad (3r_T^3 N_o) \quad (13526)$$

$$\tau^7_{\gamma,\delta,i} = \sum_{\epsilon \in A} Y^2_{i,\epsilon} \tau^6_{\gamma,\epsilon,\delta} \quad (2r_T^3 N_o) \quad (13527)$$

$$\tau^8_{\gamma,\delta,w} = \sum_{\epsilon \in A} \sum_{i \in O} {}^2D^2_{i,w} Y^{2,*}_{i,\delta} \tau^0_{\epsilon,\delta,w} \tau^7_{\gamma,\epsilon,i} \quad (4r_D r_T^3 N_o) \quad (13528)$$

$$\tau^9_{\gamma,\delta,w} = \sum_{\epsilon \in A} Z^*_{\epsilon,\delta} \tau^8_{\gamma,\epsilon,w} \quad (2r_D r_T^3) \quad (13529)$$

$$\tau^{10}_{\gamma,\delta,w} = \sum_{\epsilon \in A} Z_{\epsilon,\gamma} \tau^9_{\epsilon,\delta,w} \quad (2r_D r_T^3) \quad (13530)$$

$$\tau^{11}_{\gamma,\delta,w} = \sum_{a \in V} {}^2D^3_{a,w} Y^3_{a,\gamma} Y^{3,*}_{a,\delta} \quad (3r_D r_T^2 N_v) \quad (13531)$$

$${}^2R^4_{i,\gamma} \leftarrow \sum_{\delta \in A} \sum_{w \in D} \frac{1}{4} {}^2D^4_{i,w} Y^4_{i,\delta} \tau^{10}_{\delta,\gamma,w} \tau^{11}_{\delta,\gamma,w} \quad (4r_D r_T^2 N_o) \quad (13532)$$

Raw expression

$${}^2R^4_{j,\zeta} \leftarrow \sum_{\gamma \in A} \sum_{i \in O} \sum_{k \in O} \sum_{l \in O} \sum_{a \in V} \sum_{b \in V} \sum_{c \in V} \sum_{d \in V} \frac{1}{4} \quad (13533)$$

$$Y^{1,*}_{a,\gamma} \ Y^{2,*}_{i,\gamma} \ Z^*_{\gamma,\zeta} \ Y^{3,*}_{b,\zeta}$$

$${}^2D^{a,i,b,j} \ {}^2T_{c,k,a,l} \ {}^2T_{d,i,b,j} \ V_{k,d,l,c}$$

Factorized expression

$$\tau^0_{\gamma,\alpha} = \sum_{a \in V} W^4_{a,\alpha} Y^1_{a,\gamma} \quad (2r_T r_V N_v) \quad (13534)$$

$$\tau^1_{\gamma,\alpha,i} = \sum_{\beta \in B} X_{\alpha,\beta} W^3_{i,\beta} \tau^0_{\gamma,\beta} \quad (3r_T r_V^2 N_o) \quad (13535)$$

$$\tau^2_{\gamma,\alpha} = \sum_{i \in O} W^1_{i,\alpha} Y^2_{i,\gamma} \quad (2r_T r_V N_o) \quad (13536)$$

$$\tau^3_{\gamma,\alpha} = \sum_{\delta \in A} \sum_{i \in O} Z_{\delta,\gamma} Y^4_{i,\gamma} \tau^2_{\delta,\alpha} \tau^1_{\delta,\alpha,i} \quad (4r_T^2 r_V N_o) \quad (13537)$$

$$\tau^4_{\gamma,a} = \sum_{\alpha \in B} W^2_{a,\alpha} \tau^3_{\gamma,\alpha} \quad (2r_T r_V N_v) \quad (13538)$$

$$\tau^5_{a,b} = \sum_{\gamma \in A} Y^3_{b,\gamma} \tau^4_{\gamma,a} \quad (2r_T N_v^2) \quad (13539)$$

$$\tau^6_{\gamma,a} = \sum_{b \in V} Y^1_{b,\gamma} \tau^5_{b,a} \quad (2r_T N_v^2) \quad (13540)$$

$$\tau^7_{\gamma,\delta,w} = \sum_{a \in V} {}^2D^3_{a,w} Y^{3,*}_{a,\delta} \tau^6_{\gamma,a} \quad (3r_D r_T^2 N_v) \quad (13541)$$

$$\tau^8_{\gamma,\delta,w} = \sum_{a \in V} {}^2D^1_{a,w} Y^3_{a,\gamma} Y^{1,*}_{a,\delta} \quad (3r_D r_T^2 N_v) \quad (13542)$$

$$\tau^9_{\gamma,\delta,w} = \sum_{i \in O} {}^2D^2_{i,w} Y^4_{i,\gamma} Y^{2,*}_{i,\delta} \quad (3r_D r_T^2 N_o) \quad (13543)$$

$$\tau_{\gamma,\delta,w}^{10} = \sum_{\epsilon \in A} Z_{\epsilon,\delta}^* \tau_{\gamma,\epsilon,w}^8 \tau_{\gamma,\epsilon,w}^9 \quad (3r_D r_T^3) \quad (13544)$$

$$\tau_{\gamma,\delta,w}^{11} = \sum_{\epsilon \in A} Z_{\gamma,\epsilon} \tau_{\epsilon,\delta,w}^{10} \quad (2r_D r_T^3) \quad (13545)$$

$${}^2R_{i,\gamma}^4 \leftarrow \sum_{\delta \in A} \sum_{w \in D} \frac{1}{4} {}^2D_{i,w}^4 Y_{i,\delta}^2 \tau_{\delta,\gamma,w}^{11} \tau_{\delta,\gamma,w}^7 \quad (4r_D r_T^2 N_o) \quad (13546)$$

Raw expression

$${}^2R_{j,\zeta}^4 \leftarrow \sum_{\gamma \in A} \sum_{i \in O} \sum_{k \in O} \sum_{l \in O} \sum_{a \in V} \sum_{b \in V} \sum_{c \in V} \sum_{d \in V} \frac{1}{4} \quad (13547)$$

$$Y_{a,\gamma}^{1,*} Y_{i,\gamma}^{2,*} Z_{\gamma,\zeta}^* Y_{b,\zeta}^{3,*} {}^2D_{a,i,b,j} {}^2T_{c,k,b,l} {}^2T_{d,j,a,i} V_{k,d,l,c}$$

Factorized expression

$$\tau_{\gamma,\delta,w}^0 = \sum_{a \in V} {}^2D_{a,w}^1 Y_{a,\gamma}^3 Y_{a,\delta}^{1,*} \quad (3r_D r_T^2 N_v) \quad (13548)$$

$$\tau_{\gamma,\delta,w}^1 = \sum_{i \in O} {}^2D_{i,w}^2 Y_{i,\gamma}^4 Y_{i,\delta}^{2,*} \quad (3r_D r_T^2 N_o) \quad (13549)$$

$$\tau_{\gamma,\delta,w}^2 = \sum_{\epsilon \in A} Z_{\epsilon,\delta}^* \tau_{\gamma,\epsilon,w}^0 \tau_{\gamma,\epsilon,w}^1 \quad (3r_D r_T^3) \quad (13550)$$

$$\tau_{\gamma,\delta,w}^3 = \sum_{\epsilon \in A} Z_{\gamma,\epsilon} \tau_{\epsilon,\delta,w}^2 \quad (2r_D r_T^3) \quad (13551)$$

$$\tau_{\gamma,\alpha}^4 = \sum_{a \in V} W_{a,\alpha}^4 Y_{a,\gamma}^1 \quad (2r_T r_V N_v) \quad (13552)$$

$$\tau_{\gamma,\alpha,i}^5 = \sum_{\beta \in B} X_{\alpha,\beta} W_{i,\beta}^3 \tau_{\gamma,\beta}^4 \quad (3r_T r_V^2 N_o) \quad (13553)$$

$$\tau_{\gamma,\alpha}^6 = \sum_{i \in O} W_{i,\alpha}^1 Y_{i,\gamma}^2 \quad (2r_T r_V N_o) \quad (13554)$$

$$\tau_{\gamma,\alpha}^7 = \sum_{a \in V} W_{a,\alpha}^2 Y_{a,\gamma}^1 \quad (2r_T r_V N_v) \quad (13555)$$

$$\tau_{\gamma,\delta,i}^8 = \sum_{\alpha \in B} \tau_{\gamma,\alpha}^6 \tau_{\delta,\alpha}^7 \tau_{\gamma,\alpha,i}^5 \quad (3r_T^2 r_V N_o) \quad (13556)$$

$$\tau_{\gamma,\delta,\epsilon}^9 = \sum_{i \in O} Z_{\delta,\epsilon} Y_{i,\epsilon}^4 \tau_{\gamma,\delta,i}^8 \quad (3r_T^3 N_o) \quad (13557)$$

$$\tau_{\gamma,\delta,i}^{10} = \sum_{\epsilon \in A} Y_{i,\epsilon}^2 \tau_{\gamma,\epsilon,\delta}^9 \quad (2r_T^3 N_o) \quad (13558)$$

$$\tau_{\gamma,\delta,w}^{11} = \sum_{a \in V} {}^2D_{a,w}^3 Y_{a,\gamma}^3 Y_{a,\delta}^{3,*} \quad (3r_D r_T^2 N_v) \quad (13559)$$

$$\tau_{\gamma,\delta,w,i}^{12} = \sum_{\epsilon \in A} \tau_{\gamma,\epsilon,i}^{10} \tau_{\epsilon,\delta,w}^{11} \quad (2r_D r_T^3 N_o) \quad (13560)$$

$$\tau_{\gamma,w,i}^{13} = \sum_{\delta \in A} \tau_{\delta,\gamma,w}^3 \tau_{\delta,\gamma,w,i}^{12} \quad (2r_D r_T^2 N_o) \quad (13561)$$

$${}^2R_{i,\gamma}^4 \leftarrow \sum_{w \in D} \frac{1}{4} {}^2D_{i,w}^4 \tau_{\gamma,w,i}^{13} \quad (2r_D r_T N_o) \quad (13562)$$

## XII. ENVIRONMENT OF THE $Y^1$ FACTOR

Here expressions for the environment of the  $Y^1$  factor in the THC decomposition are given along with their cost

$$\tau_{\gamma,\delta}^0 = \sum_{i \in O} Y_{i,\gamma}^2 Y_{i,\delta}^{*,2} \quad (2r_T^2 N_o) \quad (13563)$$

$$\tau_{\gamma,\delta}^1 = \sum_{a \in V} Y_{a,\gamma}^3 Y_{a,\delta}^{*,3} \quad (2r_T^2 N_v) \quad (13564)$$

$$\tau_{\gamma,\delta}^2 = \sum_{i \in O} Y_{i,\gamma}^4 Y_{i,\delta}^{*,4} \quad (2r_T^2 N_o) \quad (13565)$$

$$\tau_{\gamma,\delta}^3 = \sum_{\epsilon \in A} Z_{\delta,\epsilon}^* \tau_{\gamma,\epsilon}^1 \tau_{\gamma,\epsilon}^2 \quad (3r_T^3) \quad (13566)$$

$$\tau_{\gamma,\delta}^4 = \sum_{\epsilon \in A} Z_{\gamma,\epsilon} \tau_{\epsilon,\delta}^3 \quad (2r_T^3) \quad (13567)$$

$$A_{\gamma,\delta}^1 = \tau_{\delta,\gamma}^0 \tau_{\delta,\gamma}^4 \quad (r_T^2) \quad (13568)$$

### XIII. ENVIRONMENT OF THE $Y^2$ FACTOR

Here expressions for the environment of the  $Y^2$  factor in the THC decomposition are given along with their cost

$$\tau^0_{\gamma,\delta} = \sum_{a \in V} Y^1_{a,\gamma} Y^{*,1}_{a,\delta} \quad (2r_T^2 N_v) \quad (13569)$$

$$\tau^1_{\gamma,\delta} = \sum_{a \in V} Y^3_{a,\gamma} Y^{*,3}_{a,\delta} \quad (2r_T^2 N_v) \quad (13570)$$

$$\tau^2_{\gamma,\delta} = \sum_{i \in O} Y^4_{i,\gamma} Y^{*,4}_{i,\delta} \quad (2r_T^2 N_o) \quad (13571)$$

$$\tau^3_{\gamma,\delta} = \sum_{\epsilon \in A} Z^*_{\delta,\epsilon} \tau^1_{\gamma,\epsilon} \tau^2_{\gamma,\epsilon} \quad (3r_T^3) \quad (13572)$$

$$\tau^4_{\gamma,\delta} = \sum_{\epsilon \in A} Z_{\gamma,\epsilon} \tau^3_{\epsilon,\delta} \quad (2r_T^3) \quad (13573)$$

$$A^2_{\gamma,\delta} = \tau^0_{\delta,\gamma} \tau^4_{\delta,\gamma} \quad (r_T^2) \quad (13574)$$

### XIV. ENVIRONMENT OF THE $Z$ FACTOR (LEFT)

Here expressions for the environment of the  $Z$  factor in the THC decomposition are given along with their cost

$$\tau^0_{\gamma,\delta} = \sum_{a \in V} Y^1_{a,\gamma} Y^{*,1}_{a,\delta} \quad (2r_T^2 N_v) \quad (13575)$$

$$\tau^1_{\gamma,\delta} = \sum_{i \in O} Y^2_{i,\gamma} Y^{*,2}_{i,\delta} \quad (2r_T^2 N_o) \quad (13576)$$

$$A^{zl}_{\gamma,\delta} = \tau^0_{\delta,\gamma} \tau^1_{\delta,\gamma} \quad (r_T^2) \quad (13577)$$

### XV. ENVIRONMENT OF THE $Z$ FACTOR (RIGHT)

Here expressions for the environment of the  $Z$  factor in the THC decomposition are given along with their cost

$$\tau^0_{\gamma,\delta} = \sum_{a \in V} Y^3_{a,\gamma} Y^{*,3}_{a,\delta} \quad (2r_T^2 N_v) \quad (13578)$$

$$\tau^1_{\gamma,\delta} = \sum_{i \in O} Y^4_{i,\gamma} Y^{*,4}_{i,\delta} \quad (2r_T^2 N_o) \quad (13579)$$

$$A^{zr}_{\gamma,\delta} = \tau^0_{\delta,\gamma} \tau^1_{\delta,\gamma} \quad (r_T^2) \quad (13580)$$

### XVI. ENVIRONMENT OF THE $Y^3$ FACTOR

Here expressions for the environment of the  $Y^3$  factor in the THC decomposition are given along with their cost

$$\tau^0_{\gamma,\delta} = \sum_{a \in V} Y^1_{a,\gamma} Y^{*,1}_{a,\delta} \quad (2r_T^2 N_v) \quad (13581)$$

$$\tau^1_{\gamma,\delta} = \sum_{i \in O} Y^2_{i,\gamma} Y^{*,2}_{i,\delta} \quad (2r_T^2 N_o) \quad (13582)$$

$$\tau^2_{\gamma,\delta} = \sum_{\epsilon \in A} Z^*_{\epsilon,\delta} \tau^0_{\gamma,\epsilon} \tau^1_{\gamma,\epsilon} \quad (3r_T^3) \quad (13583)$$

$$\tau^3_{\gamma,\delta} = \sum_{\epsilon \in A} Z_{\epsilon,\gamma} \tau^2_{\epsilon,\delta} \quad (2r_T^3) \quad (13584)$$

$$\tau^4_{\gamma,\delta} = \sum_{i \in O} Y^4_{i,\gamma} Y^{*,4}_{i,\delta} \quad (2r_T^2 N_o) \quad (13585)$$

$$A^3_{\gamma,\delta} = \tau^3_{\delta,\gamma} \tau^4_{\delta,\gamma} \quad (r_T^2) \quad (13586)$$

### XVII. ENVIRONMENT OF THE $Y^4$ FACTOR

Here expressions for the environment of the  $Y^4$  factor in the THC decomposition are given along with their cost

$$\tau^0_{\gamma,\delta} = \sum_{a \in V} Y^1_{a,\gamma} Y^{*,1}_{a,\delta} \quad (2r_T^2 N_v) \quad (13587)$$

$$\tau^1_{\gamma,\delta} = \sum_{i \in O} Y^2_{i,\gamma} Y^{*,2}_{i,\delta} \quad (2r_T^2 N_o) \quad (13588)$$

$$\tau^2_{\gamma,\delta} = \sum_{\epsilon \in A} Z^*_{\epsilon,\delta} \tau^0_{\gamma,\epsilon} \tau^1_{\gamma,\epsilon} \quad (3r_T^3) \quad (13589)$$

$$\tau^3_{\gamma,\delta} = \sum_{\epsilon \in A} Z_{\epsilon,\gamma} \tau^2_{\epsilon,\delta} \quad (2r_T^3) \quad (13590)$$

$$\tau^4_{\gamma,\delta} = \sum_{a \in V} Y^3_{a,\gamma} Y^{*,3}_{a,\delta} \quad (2r_T^2 N_v) \quad (13591)$$

$$A^4_{\gamma,\delta} = \tau^3_{\delta,\gamma} \tau^4_{\delta,\gamma} \quad (r_T^2) \quad (13592)$$



- 
- [1] K. L. Schuchardt, B. T. Didier, T. Elsethagen, L. Sun, V. Gurumoorthi, J. Chase, J. Li, and T. L. Windus, *J. Chem. Inform. Model.* **47**, 1045 (2007).
  - [2] E. G. Hohenstein, R. M. Parrish, C. D. Sherrill, and T. J. Martínez, *J. Chem. Phys.* **137**, 221101 (2012).
  - [3] J. Zhao and G. E. Scuseria, “Generic and efficient canonicalization of combinatorial objects,” <http://jz21.web.rice.edu/drudge/> (in preparation).
  - [4] J. Zhao and G. E. Scuseria, “Efficient optimization of tensor contractions, parts i and ii,” <http://jz21.web.rice.edu/gristmill/> (in preparation).
  - [5] S. v. d. Walt, S. C. Colbert, and G. Varoquaux, *Comput. Sci. Eng.* **13**, 22 (2011).
